# Supplementary material for: N$^3$LO Spin-Orbit Interaction via the EFT of Spinning Gravitating Objects
Source: arXiv:2208.14949 ancillary file (2023-01-25)
Supplement: Supplementary file 1 [file frules-field-vis.pdf]

Field propagator, time derivative insertions and vertex rules.

Position space integration (momentum space for propagators) has been suppressed.

MS-bar scheme for the gravitational coupling is  $G_d = G \left( \sqrt{4 \pi \exp(\gamma)} R_0 \right)^{d-3}$

Legends :

- 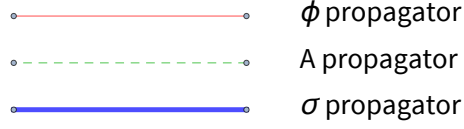  $\phi$  propagator
- 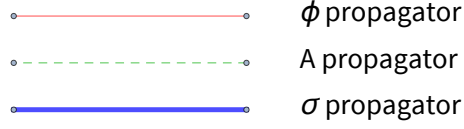 A propagator
- 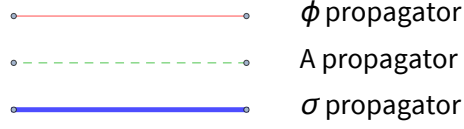  $\sigma$  propagator

$$\left\{ \text{Red line with dots} , 4 \pi G_d \frac{2 (d-2)}{d-1} \delta(t_1 - t_2) \frac{e^{i \vec{k} \cdot (\vec{x}_1 - \vec{x}_2)}}{\vec{k}^2} \right\}$$

$$\left\{ \text{Green dashed line with dots} , -16 \pi G_d \delta_{ij} \delta(t_1 - t_2) \frac{e^{i \vec{k} \cdot (\vec{x}_1 - \vec{x}_2)}}{\vec{k}^2} \right\}$$

$$\left\{ \text{Blue line with dots} , 32 \pi G_d \left( \frac{1}{2} \left( \delta_{ik} \delta_{jl} + \delta_{il} \delta_{jk} + \left( 2 - \frac{2(d-1)}{d-2} \right) \delta_{ij} \delta_{kl} \right) \right) \delta(t_1 - t_2) \frac{e^{i \vec{k} \cdot (\vec{x}_1 - \vec{x}_2)}}{\vec{k}^2} \right\}$$

$$\left\{ \text{Red line with star} , (c^{-1})^2 \frac{d-1}{2(d-2)} \frac{(\partial_t \phi)^2}{8 \pi G_d} \right\}$$

$$\left\{ \text{Green dashed line with star} , - (c^{-1})^2 \frac{(\partial_t A_i \partial_t A^i)}{32 \pi G_d} \right\}$$

$$\left\{ \text{Blue line with star} , (c^{-1})^2 \frac{2 \left( \partial_t \sigma_{ij} \partial_t \sigma^{ij} \right) - \left( \partial_t \sigma^i_i \right)^2}{128 \pi G_d} \right\}$$

$$\left\{ \text{Cross vertex} , - \frac{1}{128 (-2+d) G_d \pi} (c^{-1})^8 (-1+d) \right\}$$

$$\left( \left( \sigma^i_i \right)^2 \left( \partial_i \phi \partial^i \phi \right) - 2 \left( \sigma_{i11} \sigma^{i11} \right) \left( \partial_i \phi \partial^i \phi \right) - 4 \left( \sigma^i_i \right) \left( \sigma_{i11} \partial^i \phi \partial^{i1} \phi \right) + 8 \left( \sigma_i^{i2} \sigma_{i1i2} \partial^i \phi \partial^{i1} \phi \right) \right) \}$$

$$\left\{ \text{Three blue lines vertex} , \frac{1}{256 G_d \pi} \right\}$$

$$\begin{aligned} & (c^{-1})^8 \left( 4 \left( \sigma^{i11} \partial_i \sigma^{i2i3} \partial_{i1} \sigma_{i2i3} \right) - 2 \left( \sigma^{i11} \partial_i \sigma^{i2}_{i2} \partial_{i1} \sigma^{i3}_{i3} \right) + \left( \sigma^i_i \right) \left( \partial_{i1} \sigma^{i2}_{i2} \partial^{i1} \sigma^i_i \right) + \right. \\ & 8 \left( \sigma^{i11} \partial_{i1} \sigma^{i3}_{i3} \partial_{i2} \sigma^i_{i2} \right) + 4 \left( \sigma^i_i \right) \left( \partial_i \sigma^{i11} \partial_{i2} \sigma^{i1}_{i2} \right) - 8 \left( \sigma^{i11} \partial_{i1} \sigma^i_{i2} \partial_{i2} \sigma^{i3}_{i3} \right) - \\ & 4 \left( \sigma^{i11} \partial_{i2} \sigma^{i3}_{i3} \partial^{i2} \sigma_{i11} \right) - 4 \left( \sigma^i_i \right) \left( \partial_{i1} \sigma_{i1i2} \partial^{i2} \sigma^{i1}_{i1} \right) - 2 \left( \sigma^i_i \right) \left( \partial_{i2} \sigma_{i1i1} \partial^{i2} \sigma^{i1}_{i1} \right) - \\ & \left. 8 \left( \sigma^{i11} \partial_{i2} \sigma^i_{i2} \partial_{i3} \sigma_{i1i3} \right) + 8 \left( \sigma^{i11} \partial_{i2} \sigma_{i1i3} \partial^{i3} \sigma^i_{i2} \right) + 8 \left( \sigma^{i11} \partial_{i3} \sigma_{i1i2} \partial^{i3} \sigma^i_{i2} \right) \right) \} \end{aligned}$$

$$\left\{ \text{Three green dashed lines vertex} , \frac{(c^{-1})^6 \left( A^i \partial_i A^{i1} \partial_t A_{i1} \right)}{16 G_d \pi} \right\}$$

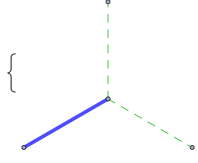

$$, \frac{1}{64 G_d \pi} (c^{-1})^6 \left( (\sigma^i_i) \left( (\partial_i A^i)^2 - (\partial_i A_{i1} \partial^{i1} A^i) + (\partial_{i1} A_i \partial^{i1} A^i) \right) - \right.$$

$$\left. \frac{2 \left( 2 (\partial_i A^i) (\sigma_{i11} \partial^{i1} A^i) + (\sigma_{i12} \partial_{i1} A^{i2} \partial^{i1} A^i) + (\sigma_{i112} \partial^{i1} A^i \partial^{i2} A_i) - 2 (\sigma_{i12} \partial^{i1} A^i \partial^{i2} A_{i1}) \right) - (c^{-1})^8 \left( (\sigma^i_i) (\partial_t A_i \partial_t A^i) - 2 (\sigma_{i11} \partial_t A^i \partial_t A^{i1}) \right) \right\}$$

$$64 G_d \pi$$

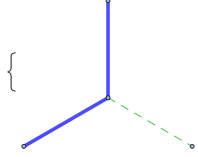

$$, \frac{1}{64 G_d \pi}$$

$$\begin{aligned} & (c^{-1})^8 \left( 2 (\sigma^{i1i2} \partial_i \sigma_{i1i2} \partial_t A^i) + 2 (\sigma_i^{i1} \partial_{i1} \sigma^{i2}_{i2} \partial_t A^i) - 4 (\sigma^{i1i2} \partial_{i2} \sigma_{i11} \partial_t A^i) - \right. \\ & 4 (\sigma_i^{i1} \partial_{i2} \sigma_{i1}^{i2} \partial_t A^i) - 2 (\partial_i A^i) (\sigma^{i11} \partial_t \sigma_{i11}) - 4 (A^i \partial_{i1} \sigma^{i1i2} \partial_t \sigma_{i12}) + 4 (\sigma_{i1}^{i2} \partial^{i1} A^i \partial_t \sigma_{i12}) + \\ & 2 (A^i \partial^{i2} \sigma^{i1}_{i1} \partial_t \sigma_{i12}) + (A^i \partial_i \sigma^{i1}_{i1}) (\partial_t \sigma^i_i) - 2 (A^i \partial_{i1} \sigma_i^{i1}) (\partial_t \sigma^i_i) - 2 (\sigma_{i11} \partial^{i1} A^i) (\partial_t \sigma^i_i) + \\ & (\sigma^i_i) (- (\partial_i \sigma^{i1}_{i1} \partial_t A^i) + 2 (\partial_{i1} \sigma_i^{i1} \partial_t A^i) - 2 (\partial^{i1} A^i \partial_t \sigma_{i11}) + (\partial_i A^i) (\partial_t \sigma^i_i)) - \\ & \left. 2 (A^i \partial_i \sigma^{i1i2} \partial_t \sigma_{i1i2}) + 4 (\sigma_i^{i2} \partial^{i1} A^i \partial_t \sigma_{i1i2}) + 4 (A^i \partial^{i2} \sigma_i^{i1} \partial_t \sigma_{i1i2}) \right\} \end{aligned}$$

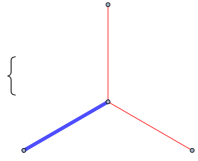

$$, - \frac{(c^{-1})^4 (-1+d) \left( (\sigma^i_i) (\partial_i \phi \partial^i \phi) - 2 (\sigma_{i11} \partial^i \phi \partial^{i1} \phi) \right)}{32 (-2+d) G_d \pi} + \frac{(c^{-1})^6 (1-d) (\sigma^i_i) (\partial_t \phi)^2}{64 G_d \pi - 32 d G_d \pi}$$

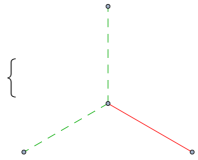

$$, \frac{(c^{-1})^4 (-1+d) \left( (\partial_i A^i)^2 - (\partial_i A_{i1} \partial^{i1} A^i) + (\partial_{i1} A_i \partial^{i1} A^i) \right) \phi}{16 (-2+d) G_d \pi}$$

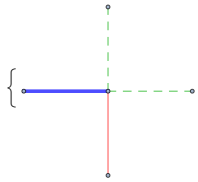

$$, \frac{1}{32 (-2+d) G_d \pi} (c^{-1})^8 (-1+d) \left( (\sigma^i_i) \left( (\partial_i A^i)^2 - (\partial_i A_{i1} \partial^{i1} A^i) + (\partial_{i1} A_i \partial^{i1} A^i) \right) - \right.$$

$$\left. 2 \left( 2 (\partial_i A^i) (\sigma_{i11} \partial^{i1} A^i) + (\sigma_{i12} \partial_{i1} A^{i2} \partial^{i1} A^i) + (\sigma_{i112} \partial^{i1} A^i \partial^{i2} A_i) - 2 (\sigma_{i12} \partial^{i1} A^i \partial^{i2} A_{i1}) \right) \right) \phi \}$$

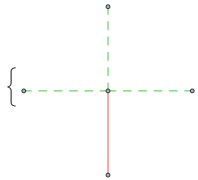

$$, \frac{(c^{-1})^8 (-1+d) \left( (\partial_i A^i) (A^i \partial_t A_i) + (A^i \partial_i A^{i1} \partial_t A_{i1}) - (A^i \partial^{i1} A_i \partial_t A_{i1}) \right) \phi}{8 (-2+d) G_d \pi}$$

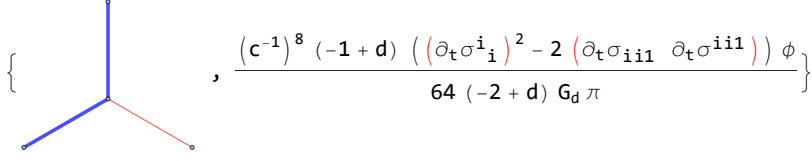

$$\left\{ , \frac{(\mathbf{c}^{-1})^8 (-1 + \mathbf{d}) \left( (\partial_{\mathbf{t}} \sigma^{\mathbf{i}}_{\mathbf{i}})^2 - 2 (\partial_{\mathbf{t}} \sigma_{\mathbf{ii1}} \partial_{\mathbf{t}} \sigma^{\mathbf{ii1}}) \right) \phi}{64 (-2 + \mathbf{d}) \mathbf{G}_{\mathbf{d}} \pi} \right\}$$

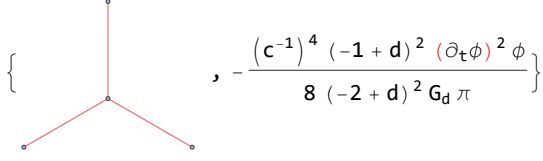

$$\left\{ , - \frac{(\mathbf{c}^{-1})^4 (-1 + \mathbf{d})^2 (\partial_{\mathbf{t}} \phi)^2 \phi}{8 (-2 + \mathbf{d})^2 \mathbf{G}_{\mathbf{d}} \pi} \right\}$$

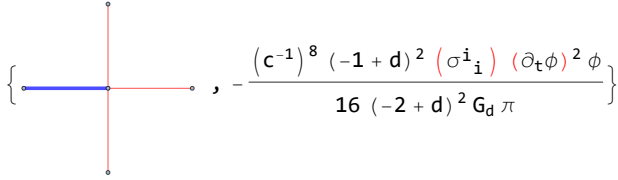

$$\left\{ , - \frac{(\mathbf{c}^{-1})^8 (-1 + \mathbf{d})^2 (\sigma^{\mathbf{i}}_{\mathbf{i}}) (\partial_{\mathbf{t}} \phi)^2 \phi}{16 (-2 + \mathbf{d})^2 \mathbf{G}_{\mathbf{d}} \pi} \right\}$$

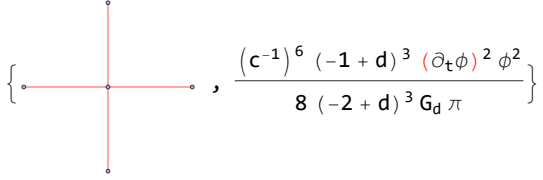

$$\left\{ , \frac{(\mathbf{c}^{-1})^6 (-1 + \mathbf{d})^3 (\partial_{\mathbf{t}} \phi)^2 \phi^2}{8 (-2 + \mathbf{d})^3 \mathbf{G}_{\mathbf{d}} \pi} \right\}$$

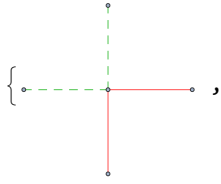

$$\left\{ , \right.$$

$$\frac{(\mathbf{c}^{-1})^8 (-1 + \mathbf{d}) (\mathbf{A}_{\mathbf{i}} \mathbf{A}^{\mathbf{i}}) (\partial_{\mathbf{t}} \phi)^2}{32 \mathbf{G}_{\mathbf{d}} \pi - 16 \mathbf{d} \mathbf{G}_{\mathbf{d}} \pi} + \frac{(\mathbf{c}^{-1})^6 (-1 + \mathbf{d})^2 \left( (\partial_{\mathbf{i}} \mathbf{A}^{\mathbf{i}})^2 - (\partial_{\mathbf{i}} \mathbf{A}_{\mathbf{ii1}} \partial^{\mathbf{ii1}} \mathbf{A}^{\mathbf{i}}) + (\partial_{\mathbf{ii1}} \mathbf{A}_{\mathbf{i}} \partial^{\mathbf{ii1}} \mathbf{A}^{\mathbf{i}}) \right) \phi^2}{16 (-2 + \mathbf{d})^2 \mathbf{G}_{\mathbf{d}} \pi} \right\}$$

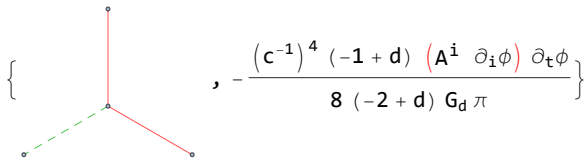

$$\left\{ , - \frac{(\mathbf{c}^{-1})^4 (-1 + \mathbf{d}) (\mathbf{A}^{\mathbf{i}} \partial_{\mathbf{i}} \phi) \partial_{\mathbf{t}} \phi}{8 (-2 + \mathbf{d}) \mathbf{G}_{\mathbf{d}} \pi} \right\}$$

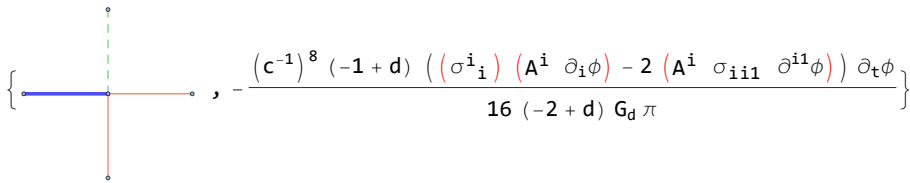

$$\left\{ , - \frac{(\mathbf{c}^{-1})^8 (-1 + \mathbf{d}) \left( (\sigma^{\mathbf{i}}_{\mathbf{i}}) (\mathbf{A}^{\mathbf{i}} \partial_{\mathbf{i}} \phi) - 2 (\mathbf{A}^{\mathbf{i}} \sigma_{\mathbf{ii1}} \partial^{\mathbf{ii1}} \phi) \right) \partial_{\mathbf{t}} \phi}{16 (-2 + \mathbf{d}) \mathbf{G}_{\mathbf{d}} \pi} \right\}$$

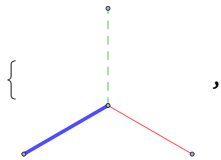

$$\left\{ , \right.$$

$$- \frac{(\mathbf{c}^{-1})^6 (-1 + \mathbf{d}) \left( -2 \left( \sigma_{\mathbf{i}\mathbf{i}\mathbf{i}} \partial^{\mathbf{i}} \phi \partial_{\mathbf{t}} \mathbf{A}^{\mathbf{i}\mathbf{1}} \right) + 2 \left( \sigma_{\mathbf{i}\mathbf{i}\mathbf{i}} \partial^{\mathbf{i}\mathbf{1}} \mathbf{A}^{\mathbf{i}} \right) \partial_{\mathbf{t}} \phi + \left( \sigma^{\mathbf{i}}_{\mathbf{i}} \right) \left( \left( \partial^{\mathbf{i}} \phi \partial_{\mathbf{t}} \mathbf{A}_{\mathbf{i}} \right) - \left( \partial_{\mathbf{i}} \mathbf{A}^{\mathbf{i}} \right) \partial_{\mathbf{t}} \phi \right) \right)}{16 (-2 + \mathbf{d}) \mathbf{G}_{\mathbf{d}} \pi} \Bigg\}$$
