# Supplementary material for: N$^3$LO Spin-Orbit Interaction via the EFT of Spinning Gravitating Objects
Source: arXiv:2208.14949 ancillary file (2023-01-25)
Supplement: Supplementary file 2 [file frules-wl-vis.pdf]

Worldline vertex rules.

Worldline time integration has been suppressed.

Spin variable presented in spin-tensor form.

Legends :

- 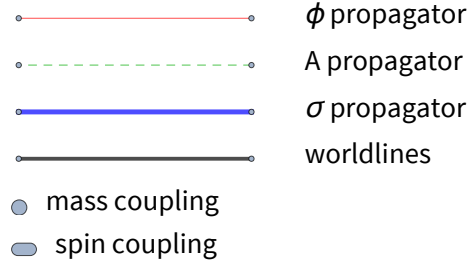  $\phi$  propagator
- 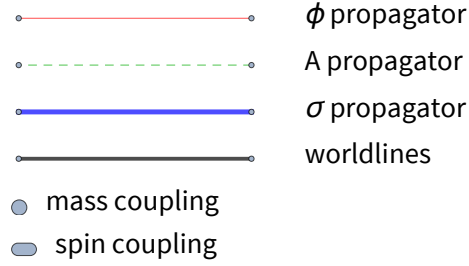 A propagator
- 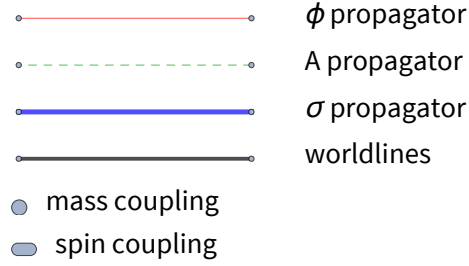  $\sigma$  propagator
- 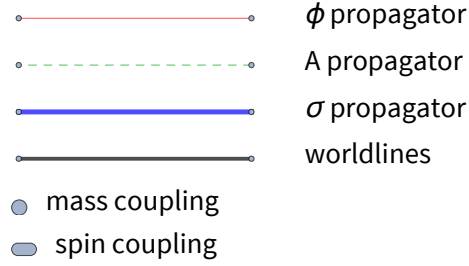 worldlines
- 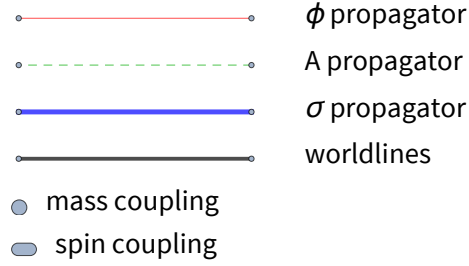 mass coupling
- 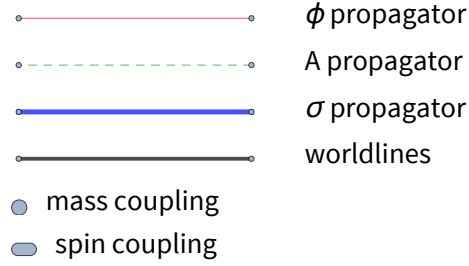 spin coupling

$$\left\{ \text{Kinetic term, } -\frac{m}{(c^{-1})^2} + \frac{1}{2} m (v_i v^i) + \frac{1}{8} (c^{-1})^2 m (v_i v^i)^2 + \right.$$

$$\left. \frac{1}{16} (c^{-1})^4 m (v_i v^i)^3 + \frac{5}{128} (c^{-1})^6 m (v_i v^i)^4 + \frac{7}{256} (c^{-1})^8 m (v_i v^i)^5 \right\}$$

$$\left\{ \text{Kinetic term, } -\frac{1}{2} (c^{-1})^3 (a^i S_{ii1} v^{i1}) - \frac{3}{8} (c^{-1})^5 (v_i v^i) (a^i S_{ii1} v^{i1}) - \right.$$

$$\left. \frac{5}{16} (c^{-1})^7 (v_i v^i)^2 (a^i S_{ii1} v^{i1}) - \frac{35}{128} (c^{-1})^9 (v_i v^i)^3 (a^i S_{ii1} v^{i1}) \right\}$$

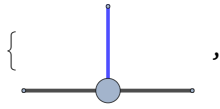

$$\frac{1}{2} (c^{-1})^4 m (v^i v^{i1} \sigma_{ii1}) + \frac{1}{4} (c^{-1})^6 m (v_i v^i) (v^i v^{i1} \sigma_{ii1}) + \frac{3}{16} (c^{-1})^8 m (v_i v^i)^2 (v^i v^{i1} \sigma_{ii1}) \left\{ \right.$$

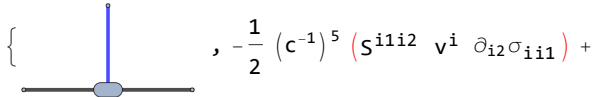

$$, -\frac{1}{2} (c^{-1})^5 (S^{i1i2} v^i \partial_{i2} \sigma_{ii1}) +$$

$$\frac{1}{4} (c^{-1})^7 \left( (a^i S_{ii1}^{i2} v^{i1} \sigma_{ii2}) - (a^i S_i^{i2} v^{i1} \sigma_{ii2}) + 2 (S_i^{i3} v^i v^{i1} v^{i2} \partial_{i2} \sigma_{ii1i3}) - \right.$$

$$\left. (S_i^{i3} v^i v^{i1} v^{i2} \partial_{i3} \sigma_{ii1i2}) + 3 (S_i^{i2} v^i v^{i1} \partial_t \sigma_{ii1i2}) \right) +$$

$$\frac{1}{16} (c^{-1})^9 \left( -6 (a^i S_{ii1} v^{i1}) (v^i v^{i1} \sigma_{ii1}) + (v_i v^i) (3 (a^i S_{ii1}^{i2} v^{i1} \sigma_{ii2}) - 3 (a^i S_i^{i2} v^{i1} \sigma_{ii2}) + \right.$$

$$\left. 6 (S_i^{i3} v^i v^{i1} v^{i2} \partial_{i2} \sigma_{ii1i3}) - 3 (S_i^{i3} v^i v^{i1} v^{i2} \partial_{i3} \sigma_{ii1i2}) + 7 (S_i^{i2} v^i v^{i1} \partial_t \sigma_{ii1i2}) \right) \left. \right\}$$

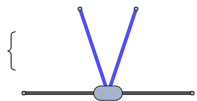

$$, \frac{1}{8} (c^{-1})^9 \left( (S^{i1i2} v^i \sigma_{ii1}^{i3} \partial_{i3} \sigma_{ii2i3}) + \right.$$

$$\left. 2 (S^{i1i2} v^i \sigma_{ii1}^{i3} \partial_{i2} \sigma_{ii3}) - 2 (S^{i1i2} v^i \sigma_{ii1}^{i3} \partial_{i3} \sigma_{ii2}) + (S^{ii1} \sigma_i^{i2} \partial_t \sigma_{ii1i2}) \right\}$$

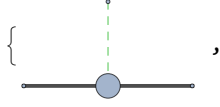

$$\left\{ (c^{-1})^2 m \left( A^i v_i \right) + \frac{1}{2} (c^{-1})^4 m \left( A^i v_i \right) \left( v_i v^i \right) + \frac{3}{8} (c^{-1})^6 m \left( A^i v_i \right) \left( v_i v^i \right)^2 + \frac{5}{16} (c^{-1})^8 m \left( A^i v_i \right) \left( v_i v^i \right)^3 \right\}$$

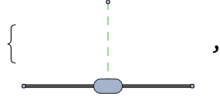

$$\begin{aligned} & -\frac{1}{2} (c^{-1})^3 \left( S_{ii1} \partial^{i1} A^i \right) + (c^{-1})^5 \left( \frac{3}{4} \left( S_{ii12} v^i v^{i1} \partial_i A^{i2} \right) - \frac{3}{4} \left( S_{ii12} v^i v^{i1} \partial^{i2} A_i \right) + \left( S_{ii1} v^i \partial_t A^{i1} \right) \right) + \\ & (c^{-1})^7 \left( - \left( A^i v_i \right) \left( a^i S_{ii1} v^{i1} \right) + \right. \\ & \quad \left. \frac{1}{16} \left( v_i v^i \right) \left( 7 \left( S_{ii12} v^i v^{i1} \partial_i A^{i2} \right) - 7 \left( S_{ii12} v^i v^{i1} \partial^{i2} A_i \right) + 8 \left( S_{ii1} v^i \partial_t A^{i1} \right) \right) \right) + \\ & \quad \frac{1}{32} (c^{-1})^9 \left( v_i v^i \right) \left( -48 \left( A^i v_i \right) \left( a^i S_{ii1} v^{i1} \right) + \right. \\ & \quad \left. \left( v_i v^i \right) \left( 11 \left( S_{ii12} v^i v^{i1} \partial_i A^{i2} \right) - 11 \left( S_{ii12} v^i v^{i1} \partial^{i2} A_i \right) + 12 \left( S_{ii1} v^i \partial_t A^{i1} \right) \right) \right) \left. \right\} \end{aligned}$$

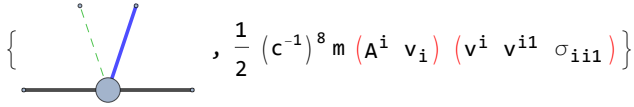

$$, \frac{1}{2} (c^{-1})^8 m \left( A^i v_i \right) \left( v^i v^{i1} \sigma_{ii1} \right) \}$$

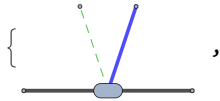

$$\begin{aligned} & \frac{1}{4} (c^{-1})^7 \left( - \left( S_{ii1}^{i2} \sigma_{ii2} \partial^{i1} A^i \right) + \left( S_i^{i2} \sigma_{ii12} \partial^{i1} A^i \right) \right) + \frac{1}{8} (c^{-1})^9 \left( -3 \left( S_{ii2}^{i3} v^i v^{i1} \sigma_{ii13} \partial_i A^{i2} \right) - \right. \\ & \quad 3 \left( S_{ii1}^{i3} v^i v^{i1} \sigma_{ii23} \partial_i A^{i2} \right) + 3 \left( S_{ii2}^{i3} v^i v^{i1} \sigma_{ii13} \partial^{i2} A_i \right) + 3 \left( S_{ii1}^{i3} v^i v^{i1} \sigma_{ii23} \partial^{i2} A_i \right) - \\ & \quad \left. 4 \left( S_{ii1}^{i2} v^i \sigma_{ii2} \partial_t A^{i1} \right) - 4 \left( S_i^{i2} v^i \sigma_{ii12} \partial_t A^{i1} \right) + 4 \left( A^i S_i^{i2} v^{i1} \partial_t \sigma_{ii12} \right) \right) \left. \right\} \end{aligned}$$

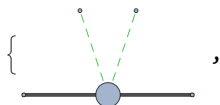

$$, \frac{1}{2} (c^{-1})^8 m \left( A^i v_i \right)^2 \left( v_i v^i \right) \}$$

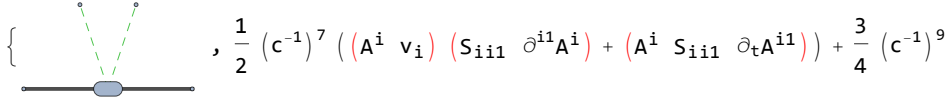

$$\left\{ , \frac{1}{2} (c^{-1})^7 \left( (A^i v_i) (S_{ii1} \partial^{i1} A^i) + (A^i S_{ii1} \partial_t A^{i1}) \right) + \frac{3}{4} (c^{-1})^9 \right.$$

$$\left. \left( (A^i S_{ii1} v^{i1}) (v^i \partial_t A_i) + (A^i v_i) \left( (S_{ii2} v^i v^{i1} \partial_i A^{i2}) - (S_{ii2} v^i v^{i1} \partial^{i2} A_i) + (S_{ii1} v^i \partial_t A^{i1}) \right) \right) \right\}$$
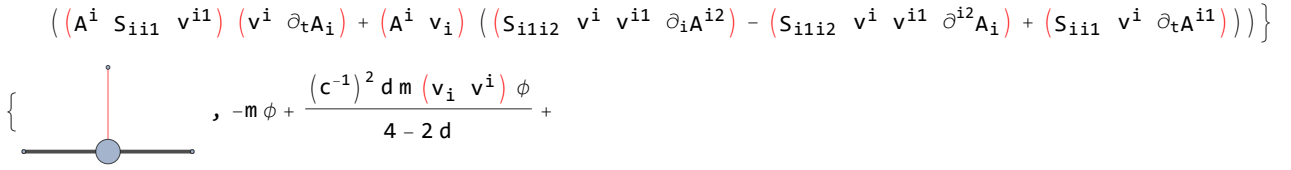

$$\left\{ , -m \phi + \frac{(c^{-1})^2 d m (v_i v^i) \phi}{4 - 2 d} + \right.$$

$$\left. \frac{(c^{-1})^4 (2 - 3 d) m (v_i v^i)^2 \phi}{8 (-2 + d)} + \frac{(c^{-1})^6 (4 - 5 d) m (v_i v^i)^3 \phi}{16 (-2 + d)} - \frac{5 (c^{-1})^8 (-6 + 7 d) m (v_i v^i)^4 \phi}{128 (-2 + d)} \right\}$$
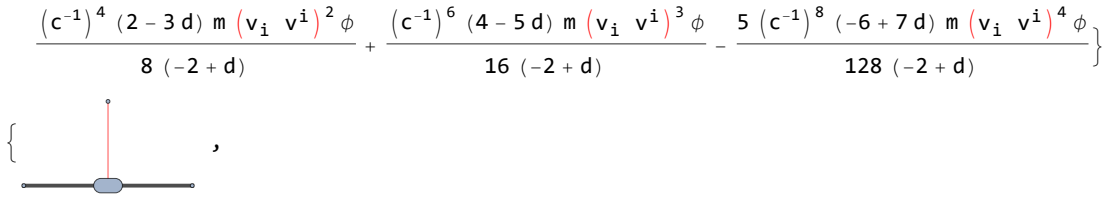

$$\left\{ , \right.$$

$$\begin{aligned} & (c^{-1})^3 \left( 1 + \frac{1}{-2 + d} \right) (S_{ii1} v^i \partial^{i1} \phi) + \frac{(c^{-1})^5 (-1 + d) \left( (v_i v^i) (S_{ii1} v^i \partial^{i1} \phi) + 2 (a^i S_{ii1} v^{i1}) \phi \right)}{2 (-2 + d)} + \\ & \frac{3 (c^{-1})^7 (-1 + d) (v_i v^i) \left( (v_i v^i) (S_{ii1} v^i \partial^{i1} \phi) + 4 (a^i S_{ii1} v^{i1}) \phi \right)}{8 (-2 + d)} + \\ & \frac{5 (c^{-1})^9 (-1 + d) (v_i v^i)^2 \left( (v_i v^i) (S_{ii1} v^i \partial^{i1} \phi) + 6 (a^i S_{ii1} v^{i1}) \phi \right)}{16 (-2 + d)} \Big\} \end{aligned}$$

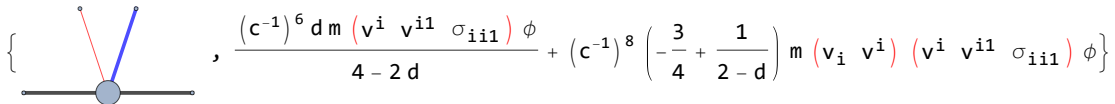

$$\left\{ , \frac{(c^{-1})^6 d m (v^i v^{i1} \sigma_{ii1}) \phi}{4 - 2 d} + (c^{-1})^8 \left( -\frac{3}{4} + \frac{1}{2 - d} \right) m (v_i v^i) (v^i v^{i1} \sigma_{ii1}) \phi \right\}$$

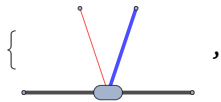

$$\left\{ , \right.$$

$$\begin{aligned} & - \frac{(c^{-1})^7 (-1 + d) \left( (S_{ii2} v^i \sigma_{ii2} \partial^{i1} \phi) + (S_{ii2} v^i \sigma_{ii2} \partial^{i1} \phi) \right)}{2 (-2 + d)} + \frac{1}{4 (-2 + d)} (c^{-1})^9 (-1 + d) \\ & \left( 2 (v^i v^{i1} \sigma_{ii1}) (S_{ii1} v^i \partial^{i1} \phi) - (v_i v^i) \left( (S_{ii2} v^i \sigma_{ii2} \partial^{i1} \phi) + (S_{ii2} v^i \sigma_{ii2} \partial^{i1} \phi) \right) + \right. \\ & \left. 2 \left( - (a^i S_{ii2} v^{i1} \sigma_{ii2}) + (a^i S_{ii2} v^{i1} \sigma_{ii2}) - 2 (S_{ii3} v^i v^{i1} v^{i2} \partial_{i2} \sigma_{ii3}) + \right. \right. \\ & \left. \left. (S_{ii3} v^i v^{i1} v^{i2} \partial_{i3} \sigma_{ii3}) - 3 (S_{ii2} v^i v^{i1} \partial_t \sigma_{ii2}) \right) \phi \right) \Big\} \end{aligned}$$

$$\left\{ \begin{array}{c} \text{Diagram: A horizontal line with a blue circle. Two red lines and one green line extend upwards from the circle.} \end{array} \right\}, (c^{-1})^4 m (A^i v_i) \phi + \frac{(c^{-1})^6 d m (A^i v_i) (v_i v^i) \phi}{4 - 2d} + \frac{(c^{-1})^8 (6 - 9d) m (A^i v_i) (v_i v^i)^2 \phi}{8 (-2 + d)} \Big\}$$

$$\left\{ \begin{array}{c} \text{Diagram: A horizontal line with a blue oval. Two red lines and one green line extend upwards from the oval.} \end{array} \right\}, -\frac{(c^{-1})^5 (-1 + d) (S_{ii1} \partial^{i1} A^i) \phi}{-2 + d} - \frac{(c^{-1})^7 (-1 + d) (A^i S_{ii1} v^{i1}) \partial_t \phi}{-2 + d} +$$

$$\frac{1}{8 (-2 + d)} (c^{-1})^9 (-1 + d) (8 (A^i v_i) ((v_i v^i) (S_{ii1} v^i \partial^{i1} \phi) + 2 (a^i S_{ii1} v^{i1}) \phi) - (v_i v^i) (7 (S_{ii2} v^i v^{i1} \partial_i A^{i2}) \phi - 7 (S_{ii2} v^i v^{i1} \partial^{i2} A_i) \phi + 8 (S_{ii1} v^i \partial_t A^{i1}) \phi + 4 (A^i S_{ii1} v^{i1}) \partial_t \phi)) \Big\}$$

$$\left\{ \begin{array}{c} \text{Diagram: A horizontal line with a blue oval. Two red lines and one blue line extend upwards from the oval.} \end{array} \right\}, -\frac{(c^{-1})^9 (-1 + d) ((S_{ii2} \sigma_{ii2} \partial^{i1} A^i) - (S_i^{i2} \sigma_{ii2} \partial^{i1} A^i)) \phi}{2 (-2 + d)} \Big\}$$

$$\left\{ \begin{array}{c} \text{Diagram: A horizontal line with a blue oval. Two red lines and two green lines extend upwards from the oval.} \end{array} \right\}, \frac{(c^{-1})^9 (-1 + d) ((A^i v_i) (S_{ii1} \partial^{i1} A^i) + (A^i S_{ii1} \partial_t A^{i1})) \phi}{-2 + d} \Big\}$$

$$\left\{ \begin{array}{c} \text{Diagram: A horizontal line with a blue circle. Two red lines extend upwards from the circle.} \end{array} \right\},$$

$$-\frac{1}{2} (c^{-1})^2 m \phi^2 + \frac{(c^{-1})^4 d^2 m (v_i v^i) \phi^2}{4 (-2 + d)^2} + \frac{(c^{-1})^6 (2 - 3d)^2 m (v_i v^i)^2 \phi^2}{16 (-2 + d)^2} + \frac{(c^{-1})^8 (4 - 5d)^2 m (v_i v^i)^3 \phi^2}{32 (-2 + d)^2} \Big\}$$

$$\left\{ \begin{array}{c} \text{Diagram: A horizontal line with a blue oval. Two red lines extend upwards from the oval.} \end{array} \right\}, -\frac{(c^{-1})^7 (-1 + d)^2 \phi ((v_i v^i) (S_{ii1} v^i \partial^{i1} \phi) + (a^i S_{ii1} v^{i1}) \phi)}{(-2 + d)^2} -$$

$$\frac{3 (c^{-1})^9 (-1 + d)^2 (v_i v^i) \phi ((v_i v^i) (S_{ii1} v^i \partial^{i1} \phi) + 2 (a^i S_{ii1} v^{i1}) \phi)}{2 (-2 + d)^2} \Big\}$$

$$\left\{ \begin{array}{c} \text{Diagram: A horizontal line with a blue circle. Two red lines and one blue line extend upwards from the circle.} \end{array} \right\}, \frac{(c^{-1})^8 d^2 m (v^i v^{i1} \sigma_{ii1}) \phi^2}{4 (-2 + d)^2} \Big\}$$

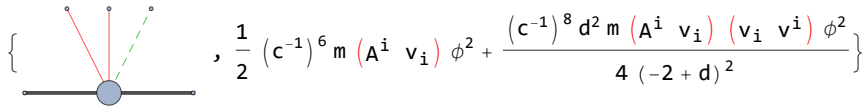

$$\left\{ , \frac{1}{2} (c^{-1})^6 m (A^i v_i) \phi^2 + \frac{(c^{-1})^8 d^2 m (A^i v_i) (v_i v^i) \phi^2}{4 (-2 + d)^2} \right\}$$

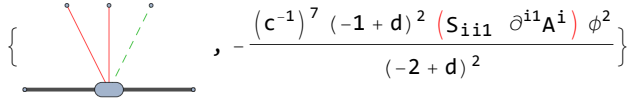

$$\left\{ , - \frac{(c^{-1})^7 (-1 + d)^2 (S_{ii1} \partial^{i1} A^i) \phi^2}{(-2 + d)^2} \right\}$$

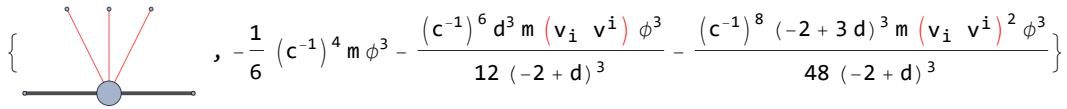

$$\left\{ , - \frac{1}{6} (c^{-1})^4 m \phi^3 - \frac{(c^{-1})^6 d^3 m (v_i v^i) \phi^3}{12 (-2 + d)^3} - \frac{(c^{-1})^8 (-2 + 3d)^3 m (v_i v^i)^2 \phi^3}{48 (-2 + d)^3} \right\}$$

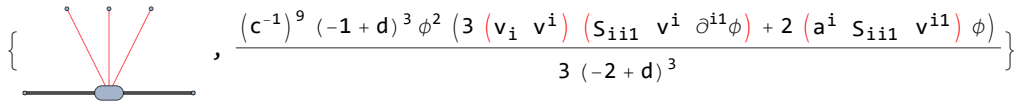

$$\left\{ , \frac{(c^{-1})^9 (-1 + d)^3 \phi^2 (3 (v_i v^i) (S_{ii1} v^i \partial^{i1} \phi) + 2 (a^i S_{ii1} v^{i1}) \phi)}{3 (-2 + d)^3} \right\}$$

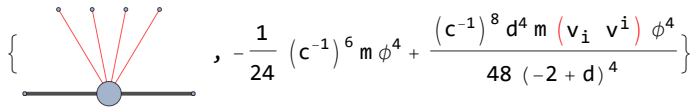

$$\left\{ , - \frac{1}{24} (c^{-1})^6 m \phi^4 + \frac{(c^{-1})^8 d^4 m (v_i v^i) \phi^4}{48 (-2 + d)^4} \right\}$$
