# Supplementary material for: N$^3$LO Spin-Orbit Interaction via the EFT of Spinning Gravitating Objects
Source: arXiv:2208.14949 ancillary file (2023-01-25)
Supplement: Supplementary file 3 [file graphs.pdf]

The diagram results are presented in MS-bar scheme.

Definitions :  $G = G_N$ ,  $\epsilon_d = d - 3$ ,  $\hat{n} = \frac{\vec{x}_1 - \vec{x}_2}{r}$ ,  $\vec{A} = d\vec{A}/dt$

Legends :

- 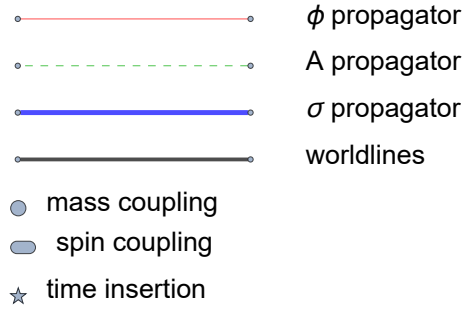  $\phi$  propagator
- 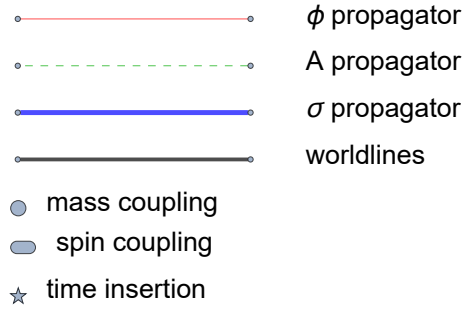 A propagator
- 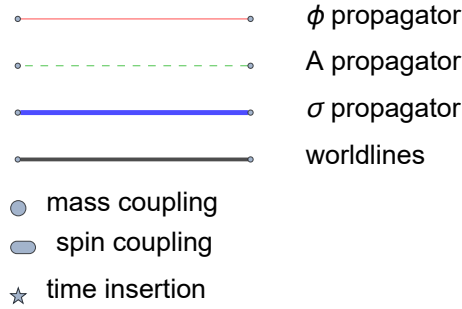  $\sigma$  propagator
- 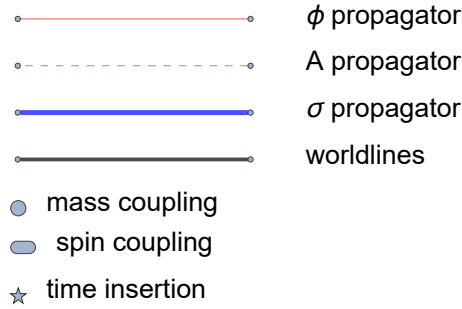 worldlines
- 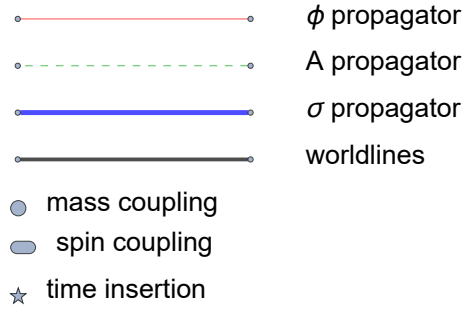 mass coupling
- 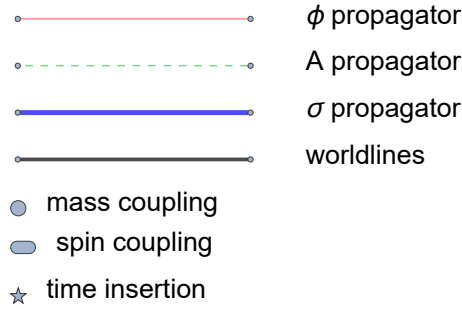 spin coupling
- 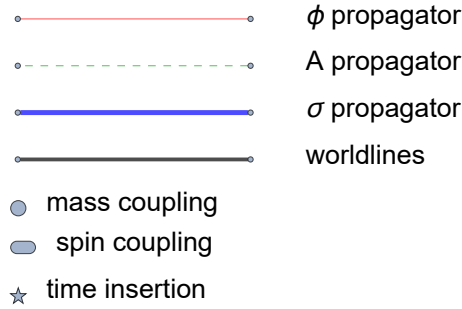 time insertion

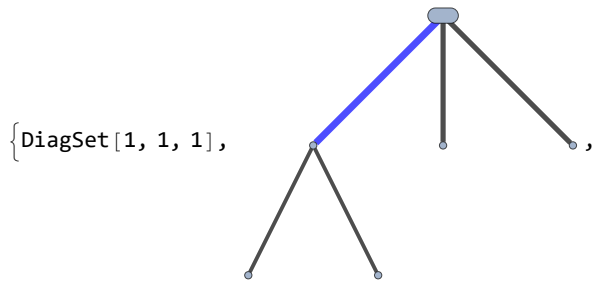

$$\begin{aligned} & \frac{1}{r} G m_2 \left( \frac{3}{2} (\vec{v}_1 \cdot \vec{v}_2)^2 \vec{S}_1 \times \vec{v}_1 \cdot \vec{a}_1 - \frac{7}{2} \vec{v}_1 \cdot \vec{v}_2 \vec{v}_1 \cdot \vec{a}_1 \vec{S}_1 \times \vec{v}_1 \cdot \vec{v}_2 - \frac{5}{2} \vec{v}_1 \cdot \vec{v}_1 \vec{v}_1 \cdot \vec{v}_2 \vec{S}_1 \times \vec{a}_1 \cdot \vec{v}_2 - \right. \\ & 2 \vec{v}_2 \cdot \vec{v}_2 \vec{v}_1 \cdot \vec{v}_2 \vec{S}_1 \times \vec{a}_1 \cdot \vec{v}_2 - (\vec{v}_2 \cdot \vec{v}_2)^2 \vec{S}_1 \times \vec{v}_1 \cdot \vec{a}_1 - \vec{v}_1 \cdot \vec{v}_1 \vec{a}_1 \cdot \vec{v}_2 \vec{S}_1 \times \vec{v}_1 \cdot \vec{v}_2 - \vec{v}_2 \cdot \vec{v}_2 \vec{a}_1 \cdot \vec{v}_2 \vec{S}_1 \times \vec{v}_1 \cdot \vec{v}_2 - \\ & \left. 3 \vec{v}_1 \cdot \vec{v}_1 \vec{v}_2 \cdot \vec{v}_2 \vec{S}_1 \times \vec{v}_1 \cdot \vec{a}_1 - \frac{7}{4} \vec{v}_1 \cdot \vec{v}_1 \vec{v}_1 \cdot \vec{v}_2 \vec{S}_1 \times \vec{v}_1 \cdot \vec{v}_2 - \frac{3}{2} \vec{v}_2 \cdot \vec{v}_2 \vec{v}_1 \cdot \vec{v}_2 \vec{S}_1 \times \vec{v}_1 \cdot \vec{v}_2 \right) + \\ & \frac{1}{r^2} G m_2 \left( -\frac{3}{4} (\vec{v}_2 \cdot \vec{v}_2)^3 \hat{n} \times \vec{S}_1 \cdot \vec{v}_1 - \frac{1}{2} \vec{v}_1 \cdot \vec{v}_1 (\vec{v}_2 \cdot \vec{v}_2)^2 \hat{n} \times \vec{S}_1 \cdot \vec{v}_1 + \frac{3}{4} \vec{v}_1 \cdot \vec{v}_2 (\vec{v}_2 \cdot \vec{v}_2)^2 \hat{n} \times \vec{S}_1 \cdot \vec{v}_2 - \right. \\ & \frac{3}{4} (\vec{v}_1 \cdot \vec{v}_1)^2 \vec{v}_2 \cdot \vec{v}_2 \hat{n} \times \vec{S}_1 \cdot \vec{v}_1 + \frac{1}{2} (\vec{v}_1 \cdot \vec{v}_2)^2 \vec{v}_2 \cdot \vec{v}_2 \hat{n} \times \vec{S}_1 \cdot \vec{v}_1 + \frac{1}{2} \vec{v}_1 \cdot \vec{v}_2 \vec{v}_2 \cdot \vec{v}_2 \hat{n} \cdot \vec{v}_1 \vec{S}_1 \times \vec{v}_1 \cdot \vec{v}_2 + \\ & \left. \frac{3}{4} \vec{v}_1 \cdot \vec{v}_1 (\vec{v}_1 \cdot \vec{v}_2)^2 \hat{n} \times \vec{S}_1 \cdot \vec{v}_1 + \frac{1}{4} \vec{v}_1 \cdot \vec{v}_1 \vec{v}_1 \cdot \vec{v}_2 \hat{n} \cdot \vec{v}_1 \vec{S}_1 \times \vec{v}_1 \cdot \vec{v}_2 \right) \} \end{aligned}$$

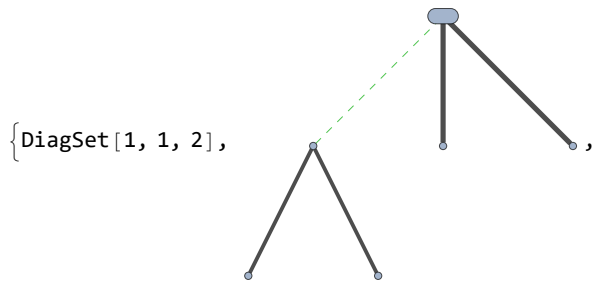

$$\begin{aligned} & \frac{1}{r} G m_2 \left( \frac{3}{2} (\vec{v}_1 \cdot \vec{v}_1)^2 \vec{S}_1 \times \vec{a}_1 \cdot \vec{v}_2 + 6 \vec{v}_1 \cdot \vec{v}_1 \vec{v}_1 \cdot \vec{a}_1 \vec{S}_1 \times \vec{v}_1 \cdot \vec{v}_2 - 6 \vec{v}_1 \cdot \vec{v}_2 \vec{v}_1 \cdot \vec{v}_1 \vec{S}_1 \times \vec{v}_1 \cdot \vec{a}_1 + \right. \\ & \vec{v}_2 \cdot \vec{v}_2 \vec{v}_1 \cdot \vec{v}_1 \vec{S}_1 \times \vec{a}_1 \cdot \vec{v}_2 + \frac{3}{2} (\vec{v}_2 \cdot \vec{v}_2)^2 \vec{S}_1 \times \vec{a}_1 \cdot \vec{v}_2 + 2 \vec{v}_2 \cdot \vec{v}_2 \vec{v}_1 \cdot \vec{a}_1 \vec{S}_1 \times \vec{v}_1 \cdot \vec{v}_2 - 2 \vec{v}_1 \cdot \vec{v}_2 \vec{v}_2 \cdot \vec{v}_2 \vec{S}_1 \times \vec{v}_1 \cdot \vec{a}_1 + \\ & \left. \frac{3}{2} (\vec{v}_1 \cdot \vec{v}_1)^2 \vec{S}_1 \times \vec{v}_1 \cdot \vec{v}_2 + \vec{v}_2 \cdot \vec{v}_2 \vec{v}_1 \cdot \vec{v}_1 \vec{S}_1 \times \vec{v}_1 \cdot \vec{v}_2 + \frac{3}{2} (\vec{v}_2 \cdot \vec{v}_2)^2 \vec{S}_1 \times \vec{v}_1 \cdot \vec{v}_2 \right) + \frac{1}{r^2} \\ & G m_2 \left( -\frac{5}{8} (\vec{v}_2 \cdot \vec{v}_2)^3 \hat{n} \times \vec{S}_1 \cdot \vec{v}_2 - \frac{3}{8} (\vec{v}_2 \cdot \vec{v}_2)^2 \hat{n} \cdot \vec{v}_1 \vec{S}_1 \times \vec{v}_1 \cdot \vec{v}_2 - \frac{9}{8} \vec{v}_1 \cdot \vec{v}_2 (\vec{v}_2 \cdot \vec{v}_2)^2 \hat{n} \times \vec{S}_1 \cdot \vec{v}_1 - \frac{1}{8} \vec{v}_1 \cdot \vec{v}_1 \vec{v}_2 \cdot \vec{v}_2 \hat{n} \cdot \vec{v}_1 \right. \end{aligned}$$

$$\vec{S}_1 \times \vec{v}_1 \cdot \vec{v}_2 - \frac{7}{8} \vec{v}_1 \cdot \vec{v}_1 \vec{v}_1 \cdot \vec{v}_2 \vec{v}_2 \cdot \vec{v}_2 \hat{n} \times \vec{S}_1 \cdot \vec{v}_1 - \frac{1}{8} (\vec{v}_1 \cdot \vec{v}_1)^2 \hat{n} \cdot \vec{v}_1 \vec{S}_1 \times \vec{v}_1 \cdot \vec{v}_2 - \frac{11}{8} (\vec{v}_1 \cdot \vec{v}_1)^2 \vec{v}_1 \cdot \vec{v}_2 \hat{n} \times \vec{S}_1 \cdot \vec{v}_1 \Big\}$$

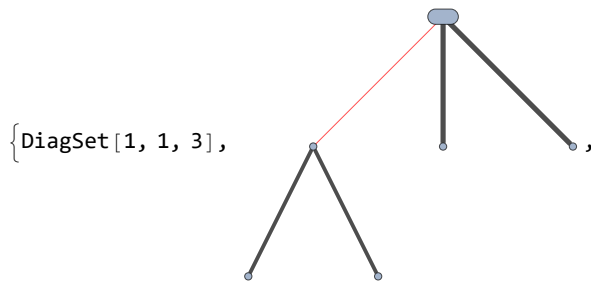

$$\frac{1}{r} G m_2 \left( \frac{15}{4} (\vec{v}_1 \cdot \vec{v}_1)^2 \vec{S}_1 \times \vec{v}_1 \cdot \vec{a}_1 + \frac{9}{2} \vec{v}_2 \cdot \vec{v}_2 \vec{v}_1 \cdot \vec{v}_1 \vec{S}_1 \times \vec{v}_1 \cdot \vec{a}_1 + \frac{7}{4} (\vec{v}_2 \cdot \vec{v}_2)^2 \vec{S}_1 \times \vec{v}_1 \cdot \vec{a}_1 \right) + \frac{1}{r^2} G m_2 \left( \frac{5}{8} (\vec{v}_1 \cdot \vec{v}_1)^3 \hat{n} \times \vec{S}_1 \cdot \vec{v}_1 + \frac{9}{8} \vec{v}_2 \cdot \vec{v}_2 (\vec{v}_1 \cdot \vec{v}_1)^2 \hat{n} \times \vec{S}_1 \cdot \vec{v}_1 + \frac{7}{8} (\vec{v}_2 \cdot \vec{v}_2)^2 \vec{v}_1 \cdot \vec{v}_1 \hat{n} \times \vec{S}_1 \cdot \vec{v}_1 + \frac{11}{8} (\vec{v}_2 \cdot \vec{v}_2)^3 \hat{n} \times \vec{S}_1 \cdot \vec{v}_1 \right) \Big\}$$

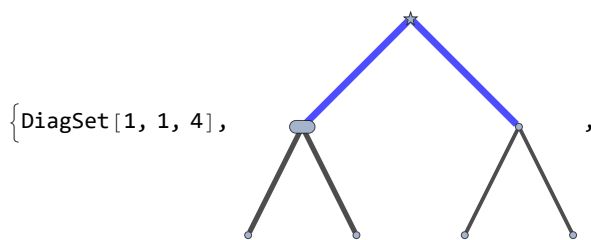

$$\begin{aligned} & G r \left( \vec{S}_1 \times \vec{v}_1 \cdot \vec{v}_2 \vec{a}_1 \cdot \vec{a}_2 + \vec{S}_1 \times \vec{v}_1 \cdot \vec{a}_2 \vec{a}_1 \cdot \vec{v}_2 + \frac{5}{2} \vec{S}_1 \times \vec{v}_1 \cdot \vec{v}_2 \vec{a}_1 \cdot \vec{a}_2 + 3 \vec{S}_1 \times \vec{a}_1 \cdot \vec{v}_2 \vec{a}_1 \cdot \vec{a}_2 + \frac{5}{2} \vec{S}_1 \times \vec{v}_1 \cdot \vec{a}_2 \vec{a}_1 \cdot \vec{v}_2 + \right. \\ & 3 \vec{S}_1 \times \vec{a}_1 \cdot \vec{a}_2 \vec{a}_1 \cdot \vec{v}_2 + \frac{7}{2} \vec{S}_1 \times \vec{a}_1 \cdot \vec{v}_2 \vec{v}_1 \cdot \vec{a}_2 + \frac{3}{2} \vec{S}_1 \times \vec{v}_1 \cdot \vec{v}_2 \vec{v}_1 \cdot \vec{a}_2 + 2 \vec{S}_1 \times \vec{a}_1 \cdot \vec{v}_2 \vec{v}_1 \cdot \vec{a}_2 + \frac{7}{2} \vec{S}_1 \times \vec{a}_1 \cdot \vec{a}_2 \vec{v}_1 \cdot \vec{v}_2 + \\ & \left. \frac{3}{2} \vec{S}_1 \times \vec{v}_1 \cdot \vec{a}_2 \vec{v}_1 \cdot \vec{v}_2 + 2 \vec{S}_1 \times \vec{a}_1 \cdot \vec{a}_2 \vec{v}_1 \cdot \vec{v}_2 + 2 \vec{S}_1 \times \vec{v}_1 \cdot \vec{a}_1 \vec{v}_2 \cdot \vec{a}_2 + 2 \vec{S}_1 \times \vec{v}_1 \cdot \vec{a}_1 \vec{v}_2 \cdot \vec{a}_2 \right) m_2 + \\ & G \left( - (\vec{S}_1 \times \vec{v}_1 \cdot \vec{v}_2) \hat{n} \cdot \vec{v}_2 \vec{a}_1 \cdot \vec{v}_2 + \frac{3}{2} \vec{S}_1 \times \vec{v}_1 \cdot \vec{v}_2 \hat{n} \cdot \vec{v}_1 \vec{a}_1 \cdot \vec{a}_2 + \frac{3}{2} \vec{S}_1 \times \vec{v}_1 \cdot \vec{a}_2 \hat{n} \cdot \vec{v}_1 \vec{a}_1 \cdot \vec{v}_2 - \frac{5}{2} \vec{S}_1 \times \vec{v}_1 \cdot \vec{v}_2 \hat{n} \cdot \vec{v}_2 \vec{a}_1 \cdot \vec{v}_2 - \right. \\ & 3 \vec{S}_1 \times \vec{a}_1 \cdot \vec{v}_2 \hat{n} \cdot \vec{v}_2 \vec{a}_1 \cdot \vec{v}_2 + \frac{1}{2} \vec{S}_1 \times \vec{v}_1 \cdot \vec{v}_2 \hat{n} \cdot \vec{a}_1 \vec{v}_1 \cdot \vec{a}_2 + 2 \vec{S}_1 \times \vec{v}_1 \cdot \vec{v}_2 \hat{n} \cdot \vec{v}_1 \vec{v}_1 \cdot \vec{a}_2 + \frac{5}{2} \vec{S}_1 \times \vec{a}_1 \cdot \vec{v}_2 \hat{n} \cdot \vec{v}_1 \vec{v}_1 \cdot \vec{a}_2 + \\ & \hat{n} \times \vec{S}_1 \cdot \vec{v}_1 \vec{a}_1 \cdot \vec{v}_2 \vec{v}_1 \cdot \vec{a}_2 + \frac{1}{2} \vec{S}_1 \times \vec{v}_1 \cdot \vec{a}_2 \hat{n} \cdot \vec{a}_1 \vec{v}_1 \cdot \vec{v}_2 + 2 \vec{S}_1 \times \vec{v}_1 \cdot \vec{a}_2 \hat{n} \cdot \vec{v}_1 \vec{v}_1 \cdot \vec{v}_2 + \frac{5}{2} \vec{S}_1 \times \vec{a}_1 \cdot \vec{a}_2 \hat{n} \cdot \vec{v}_1 \vec{v}_1 \cdot \vec{v}_2 - \\ & \frac{7}{2} \vec{S}_1 \times \vec{a}_1 \cdot \vec{v}_2 \hat{n} \cdot \vec{v}_2 \vec{v}_1 \cdot \vec{v}_2 - \frac{3}{2} \vec{S}_1 \times \vec{v}_1 \cdot \vec{v}_2 \hat{n} \cdot \vec{v}_2 \vec{v}_1 \cdot \vec{v}_2 - 2 \vec{S}_1 \times \vec{a}_1 \cdot \vec{v}_2 \hat{n} \cdot \vec{v}_2 \vec{v}_1 \cdot \vec{v}_2 + \hat{n} \times \vec{S}_1 \cdot \vec{v}_1 \vec{a}_1 \cdot \vec{a}_2 \vec{v}_1 \cdot \vec{v}_2 + \\ & \hat{n} \times \vec{S}_1 \cdot \vec{v}_1 \vec{v}_1 \cdot \vec{a}_2 \vec{v}_1 \cdot \vec{v}_2 + \hat{n} \times \vec{S}_1 \cdot \vec{a}_1 \vec{v}_1 \cdot \vec{a}_2 \vec{v}_1 \cdot \vec{v}_2 + 2 \vec{S}_1 \times \vec{v}_1 \cdot \vec{a}_1 \hat{n} \cdot \vec{v}_1 \vec{v}_2 \cdot \vec{a}_2 + \hat{n} \times \vec{S}_1 \cdot \vec{v}_2 \vec{a}_1 \cdot \vec{v}_2 \vec{v}_2 \cdot \vec{a}_2 - \\ & 2 \hat{n} \times \vec{S}_1 \cdot \vec{v}_1 \vec{v}_1 \cdot \vec{a}_1 \vec{v}_2 \cdot \vec{a}_2 - \hat{n} \times \vec{S}_1 \cdot \vec{v}_1 \vec{v}_1 \cdot \vec{v}_1 \vec{v}_2 \cdot \vec{a}_2 - \hat{n} \times \vec{S}_1 \cdot \vec{a}_1 \vec{v}_1 \cdot \vec{v}_1 \vec{v}_2 \cdot \vec{a}_2 + \hat{n} \times \vec{S}_1 \cdot \vec{v}_2 \vec{v}_1 \cdot \vec{v}_2 \vec{v}_2 \cdot \vec{a}_2 - \\ & \frac{1}{\vec{S}_1 \times \vec{v}_1 \cdot \vec{a}_1} \hat{n} \cdot \vec{v}_2 \vec{v}_2 \cdot \vec{v}_2 - \vec{S}_1 \times \vec{v}_1 \cdot \frac{1}{\vec{a}_1} \hat{n} \cdot \vec{v}_2 \vec{v}_2 \cdot \vec{v}_2 + \frac{1}{2} \hat{n} \times \vec{S}_1 \cdot \vec{v}_2 \vec{a}_1 \cdot \vec{a}_2 \vec{v}_2 \cdot \vec{v}_2 + \frac{1}{2} \hat{n} \times \vec{S}_1 \cdot \vec{a}_2 \vec{a}_1 \cdot \vec{v}_2 \vec{v}_2 \cdot \vec{v}_2 + \\ & \left. \frac{1}{2} \hat{n} \times \vec{S}_1 \cdot \vec{v}_2 \vec{v}_1 \cdot \vec{a}_2 \vec{v}_2 \cdot \vec{v}_2 + \frac{1}{2} \hat{n} \times \vec{S}_1 \cdot \vec{a}_2 \vec{v}_1 \cdot \vec{v}_2 \vec{v}_2 \cdot \vec{v}_2 - 2 \hat{n} \times \vec{S}_1 \cdot \vec{v}_1 \vec{v}_2 \cdot \vec{a}_2 \vec{v}_2 \cdot \vec{v}_2 - 2 \hat{n} \times \vec{S}_1 \cdot \vec{a}_1 \vec{v}_2 \cdot \vec{a}_2 \vec{v}_2 \cdot \vec{v}_2 \right) m_2 + \\ & \frac{1}{r} G \left( - \frac{1}{2} \vec{S}_1 \times \vec{v}_1 \cdot \vec{v}_2 \vec{v}_1 \cdot \vec{a}_2 (\hat{n} \cdot \vec{v}_1)^2 - \frac{1}{2} \vec{S}_1 \times \vec{v}_1 \cdot \vec{a}_2 \vec{v}_1 \cdot \vec{v}_2 (\hat{n} \cdot \vec{v}_1)^2 + \frac{3}{2} \vec{S}_1 \times \vec{v}_1 \cdot \vec{v}_2 \hat{n} \cdot \vec{v}_2 \vec{a}_1 \cdot \vec{v}_2 \hat{n} \cdot \vec{v}_1 + \right. \\ & 2 \vec{S}_1 \times \vec{v}_1 \cdot \vec{v}_2 \hat{n} \cdot \vec{v}_2 \vec{v}_1 \cdot \vec{v}_2 \hat{n} \cdot \vec{v}_1 + \frac{5}{2} \vec{S}_1 \times \vec{a}_1 \cdot \vec{v}_2 \hat{n} \cdot \vec{v}_2 \vec{v}_1 \cdot \vec{v}_2 \hat{n} \cdot \vec{v}_1 - \hat{n} \times \vec{S}_1 \cdot \vec{v}_1 \vec{v}_1 \cdot \vec{a}_2 \vec{v}_1 \cdot \vec{v}_2 \hat{n} \cdot \vec{v}_1 + \\ & \hat{n} \times \vec{S}_1 \cdot \vec{v}_1 \vec{v}_1 \cdot \vec{v}_1 \vec{v}_2 \cdot \vec{a}_2 \hat{n} \cdot \vec{v}_1 - \hat{n} \times \vec{S}_1 \cdot \vec{v}_2 \vec{v}_1 \cdot \vec{v}_2 \vec{v}_2 \cdot \vec{a}_2 \hat{n} \cdot \vec{v}_1 + \vec{S}_1 \times \vec{v}_1 \cdot \vec{a}_1 \hat{n} \cdot \vec{v}_2 \vec{v}_2 \cdot \vec{v}_2 \hat{n} \cdot \vec{v}_1 - \\ & \left. \frac{1}{2} \hat{n} \times \vec{S}_1 \cdot \vec{v}_2 \vec{v}_1 \cdot \vec{a}_2 \vec{v}_2 \cdot \vec{v}_2 \hat{n} \cdot \vec{v}_1 - \frac{1}{2} \hat{n} \times \vec{S}_1 \cdot \vec{a}_2 \vec{v}_1 \cdot \vec{v}_2 \vec{v}_2 \cdot \vec{v}_2 \hat{n} \cdot \vec{v}_1 + 2 \hat{n} \times \vec{S}_1 \cdot \vec{v}_1 \vec{v}_2 \cdot \vec{a}_2 \vec{v}_2 \cdot \vec{v}_2 \hat{n} \cdot \vec{v}_1 - \right. \end{aligned}$$







[illegible]

$$\frac{1}{4} \hat{n} \times \vec{S}_1 \cdot \vec{v}_1 \vec{v}_1 \cdot \vec{v}_1 (\vec{v}_2 \cdot \vec{v}_2)^2 - \frac{15}{4} \hat{n} \times \vec{S}_1 \cdot \vec{v}_1 (\hat{n} \cdot \vec{v}_1)^2 (\hat{n} \cdot \vec{v}_2)^2 \vec{v}_2 \cdot \vec{v}_2 + \frac{3}{2} \vec{S}_1 \times \vec{v}_1 \cdot \vec{v}_2 (\hat{n} \cdot \vec{v}_1)^2 \hat{n} \cdot \vec{v}_2 \vec{v}_2 \cdot \vec{v}_2 + \frac{3}{4} \hat{n} \times \vec{S}_1 \cdot \vec{v}_1 (\hat{n} \cdot \vec{v}_2)^2 \vec{v}_1 \cdot \vec{v}_1 \vec{v}_2 \cdot \vec{v}_2 - \frac{1}{2} \vec{S}_1 \times \vec{v}_1 \cdot \vec{v}_2 \hat{n} \cdot \vec{v}_2 \vec{v}_1 \cdot \vec{v}_1 \vec{v}_2 \cdot \vec{v}_2 \Big) m_2 \Big\}$$

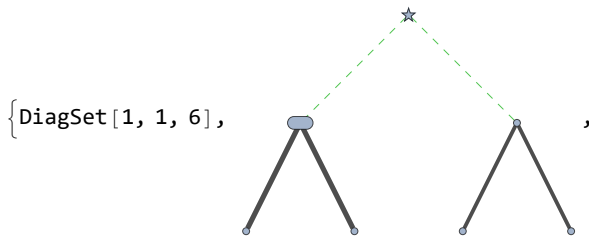

[illegible]

$$\begin{aligned} & \frac{7}{8} \hat{n} \times \vec{S}_1 \cdot \vec{v}_1 \hat{n} \cdot \vec{v}_2 \vec{v}_1 \cdot \vec{v}_1 \vec{v}_1 \cdot \vec{v}_2 - \frac{7}{8} \hat{n} \times \vec{S}_1 \cdot \vec{a}_1 \hat{n} \cdot \vec{v}_2 \vec{v}_1 \cdot \vec{v}_1 \vec{v}_1 \cdot \vec{v}_2 - \frac{1}{2} \vec{S}_1 \times \vec{v}_1 \cdot \vec{v}_2 \vec{v}_1 \cdot \vec{v}_1 \vec{v}_2 \cdot \vec{a}_2 - \\ & \frac{1}{4} \vec{S}_1 \times \vec{v}_1 \cdot \vec{v}_2 \hat{n} \cdot \vec{a}_1 \hat{n} \cdot \vec{v}_2 \vec{v}_2 \cdot \vec{v}_2 + \vec{S}_1 \times \vec{v}_1 \cdot \vec{v}_2 \vec{a}_1 \cdot \vec{v}_2 \vec{v}_2 \cdot \vec{v}_2 - \frac{3}{4} \hat{n} \times \vec{S}_1 \cdot \vec{v}_1 \hat{n} \cdot \vec{v}_2 \vec{a}_1 \cdot \vec{v}_2 \vec{v}_2 \cdot \vec{v}_2 - \\ & \frac{1}{4} \vec{S}_1 \times \vec{v}_1 \cdot \vec{a}_2 \vec{v}_1 \cdot \vec{v}_1 \vec{v}_2 \cdot \vec{v}_2 + 2 \vec{S}_1 \times \vec{v}_1 \cdot \vec{v}_2 \vec{v}_1 \cdot \vec{v}_2 \vec{v}_2 \cdot \vec{v}_2 + 2 \vec{S}_1 \times \vec{a}_1 \cdot \vec{v}_2 \vec{v}_1 \cdot \vec{v}_2 \vec{v}_2 \cdot \vec{v}_2 - \\ & \frac{3}{4} \hat{n} \times \vec{S}_1 \cdot \vec{v}_1 \hat{n} \cdot \vec{v}_2 \vec{v}_1 \cdot \vec{v}_2 \vec{v}_2 \cdot \vec{v}_2 - \frac{3}{4} \hat{n} \times \vec{S}_1 \cdot \vec{a}_1 \hat{n} \cdot \vec{v}_2 \vec{v}_1 \cdot \vec{v}_2 \vec{v}_2 \cdot \vec{v}_2 + \frac{3}{2} \vec{S}_1 \times \vec{v}_1 \cdot \vec{v}_2 \vec{v}_2 \cdot \vec{a}_2 \vec{v}_2 \cdot \vec{v}_2 \Big) m_2 + \frac{1}{r^2} \\ G & \left( \frac{3}{8} \vec{S}_1 \times \vec{v}_1 \cdot \vec{v}_2 \hat{n} \cdot \vec{v}_2 \vec{v}_1 \cdot \vec{v}_1 (\hat{n} \cdot \vec{v}_1)^2 + \frac{3}{4} \vec{S}_1 \times \vec{v}_1 \cdot \vec{v}_2 \hat{n} \cdot \vec{v}_2 \vec{v}_2 \cdot \vec{v}_2 (\hat{n} \cdot \vec{v}_1)^2 + \frac{9}{8} \hat{n} \times \vec{S}_1 \cdot \vec{v}_2 \hat{n} \cdot \vec{v}_2 (\vec{v}_2 \cdot \vec{v}_2)^2 \hat{n} \cdot \vec{v}_1 - \right. \\ & \frac{9}{8} \vec{S}_1 \times \vec{v}_1 \cdot \vec{v}_2 \vec{v}_1 \cdot \vec{v}_1 \vec{v}_1 \cdot \vec{v}_2 \hat{n} \cdot \vec{v}_1 + \frac{21}{8} \hat{n} \times \vec{S}_1 \cdot \vec{v}_1 \hat{n} \cdot \vec{v}_2 \vec{v}_1 \cdot \vec{v}_1 \vec{v}_1 \cdot \vec{v}_2 \hat{n} \cdot \vec{v}_1 - \\ & \frac{5}{4} \vec{S}_1 \times \vec{v}_1 \cdot \vec{v}_2 \vec{v}_1 \cdot \vec{v}_2 \vec{v}_2 \cdot \vec{v}_2 \hat{n} \cdot \vec{v}_1 + \frac{9}{4} \hat{n} \times \vec{S}_1 \cdot \vec{v}_1 \hat{n} \cdot \vec{v}_2 \vec{v}_1 \cdot \vec{v}_2 \vec{v}_2 \cdot \vec{v}_2 \hat{n} \cdot \vec{v}_1 - \\ & \frac{1}{8} \vec{S}_1 \times \vec{v}_1 \cdot \vec{v}_2 \hat{n} \cdot \vec{v}_2 (\vec{v}_1 \cdot \vec{v}_1)^2 - \frac{7}{8} \hat{n} \times \vec{S}_1 \cdot \vec{v}_1 \vec{v}_1 \cdot \vec{v}_1 (\vec{v}_1 \cdot \vec{v}_2)^2 + \frac{3}{8} \vec{S}_1 \times \vec{v}_1 \cdot \vec{v}_2 \hat{n} \cdot \vec{v}_2 (\vec{v}_2 \cdot \vec{v}_2)^2 - \\ & \left. \frac{3}{8} \hat{n} \times \vec{S}_1 \cdot \vec{v}_2 \vec{v}_1 \cdot \vec{v}_2 (\vec{v}_2 \cdot \vec{v}_2)^2 - \frac{3}{4} \hat{n} \times \vec{S}_1 \cdot \vec{v}_1 (\vec{v}_1 \cdot \vec{v}_2)^2 \vec{v}_2 \cdot \vec{v}_2 - \frac{1}{4} \vec{S}_1 \times \vec{v}_1 \cdot \vec{v}_2 \hat{n} \cdot \vec{v}_2 \vec{v}_1 \cdot \vec{v}_1 \vec{v}_2 \cdot \vec{v}_2 \right) m_2 \Big\} \end{aligned}$$

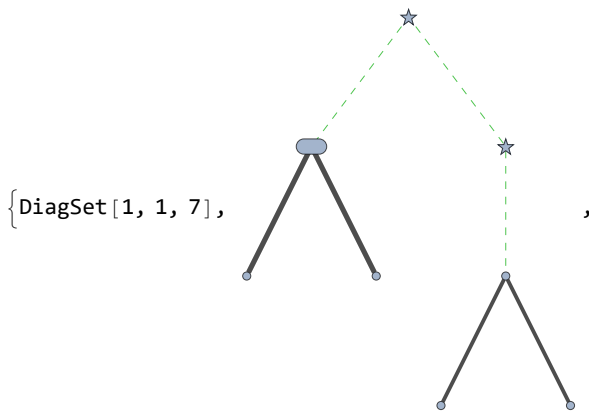

[illegible]

[illegible]

[illegible]

[illegible]



$$G \left( \frac{1}{12} \vec{S}_1 \times \vec{v}_2 \cdot \frac{1}{\vec{a}_2} (\hat{n} \cdot \vec{v}_1)^3 + \frac{1}{8} \hat{n} \times \vec{S}_1 \cdot \vec{v}_2 \hat{n} \cdot \frac{1}{\vec{a}_2} (\hat{n} \cdot \vec{v}_1)^3 + \frac{3}{8} \hat{n} \times \vec{S}_1 \cdot \vec{a}_2 \hat{n} \cdot \vec{a}_2 (\hat{n} \cdot \vec{v}_1)^3 + \frac{3}{8} \hat{n} \times \vec{S}_1 \cdot \frac{1}{\vec{a}_2} \hat{n} \cdot \vec{v}_2 (\hat{n} \cdot \vec{v}_1)^3 - \right.$$



[illegible]

$$G \left( \frac{35}{8} \hat{n} \times \vec{S_1} \cdot \vec{v_2} (\hat{n} \cdot \vec{v_2})^3 (\hat{n} \cdot \vec{v_1})^3 - \frac{15}{8} \hat{n} \times \vec{S_1} \cdot \vec{v_2} \hat{n} \cdot \vec{v_2} \vec{v_2} \cdot \vec{v_2} (\hat{n} \cdot \vec{v_1})^3 + \frac{15}{8} \vec{S_1} \times \vec{v_1} \cdot \vec{v_2} (\hat{n} \cdot \vec{v_2})^3 (\hat{n} \cdot \vec{v_1})^2 - \right. \\ \left. \frac{45}{8} \hat{n} \times \vec{S_1} \cdot \vec{v_2} (\hat{n} \cdot \vec{v_2})^2 \vec{v_1} \cdot \vec{v_2} (\hat{n} \cdot \vec{v_1})^2 - \frac{9}{8} \vec{S_1} \times \vec{v_1} \cdot \vec{v_2} \hat{n} \cdot \vec{v_2} \vec{v_2} \cdot \vec{v_2} (\hat{n} \cdot \vec{v_1})^2 + \right. \\ \left. \frac{9}{8} \hat{n} \times \vec{S_1} \cdot \vec{v_2} \vec{v_1} \cdot \vec{v_2} \vec{v_2} \cdot \vec{v_2} (\hat{n} \cdot \vec{v_1})^2 + \frac{9}{4} \hat{n} \times \vec{S_1} \cdot \vec{v_2} \hat{n} \cdot \vec{v_2} (\vec{v_1} \cdot \vec{v_2})^2 \hat{n} \cdot \vec{v_1} - \frac{15}{8} \hat{n} \times \vec{S_1} \cdot \vec{v_2} (\hat{n} \cdot \vec{v_2})^3 \vec{v_1} \cdot \vec{v_1} \hat{n} \cdot \vec{v_1} - \right. \\ \left. \frac{9}{4} \vec{S_1} \times \vec{v_1} \cdot \vec{v_2} (\hat{n} \cdot \vec{v_2})^2 \vec{v_1} \cdot \vec{v_2} \hat{n} \cdot \vec{v_1} + \frac{9}{8} \hat{n} \times \vec{S_1} \cdot \vec{v_2} \hat{n} \cdot \vec{v_2} \vec{v_1} \cdot \vec{v_1} \vec{v_2} \cdot \vec{v_2} \hat{n} \cdot \vec{v_1} + \frac{3}{4} \vec{S_1} \times \vec{v_1} \cdot \vec{v_2} \vec{v_1} \cdot \vec{v_2} \vec{v_2} \cdot \vec{v_2} \hat{n} \cdot \vec{v_1} - \right. \\ \left. \frac{1}{4} \hat{n} \times \vec{S_1} \cdot \vec{v_2} (\vec{v_1} \cdot \vec{v_2})^3 + \frac{3}{4} \vec{S_1} \times \vec{v_1} \cdot \vec{v_2} \hat{n} \cdot \vec{v_2} (\vec{v_1} \cdot \vec{v_2})^2 - \frac{3}{8} \vec{S_1} \times \vec{v_1} \cdot \vec{v_2} (\hat{n} \cdot \vec{v_2})^3 \vec{v_1} \cdot \vec{v_1} + \right. \\ \left. \frac{9}{8} \hat{n} \times \vec{S_1} \cdot \vec{v_2} (\hat{n} \cdot \vec{v_2})^2 \vec{v_1} \cdot \vec{v_1} \vec{v_1} \cdot \vec{v_2} + \frac{3}{8} \vec{S_1} \times \vec{v_1} \cdot \vec{v_2} \hat{n} \cdot \vec{v_2} \vec{v_1} \cdot \vec{v_1} \vec{v_2} \cdot \vec{v_2} - \frac{3}{8} \hat{n} \times \vec{S_1} \cdot \vec{v_2} \vec{v_1} \cdot \vec{v_1} \vec{v_1} \cdot \vec{v_2} \vec{v_2} \cdot \vec{v_2} \right) m_2 \}$$

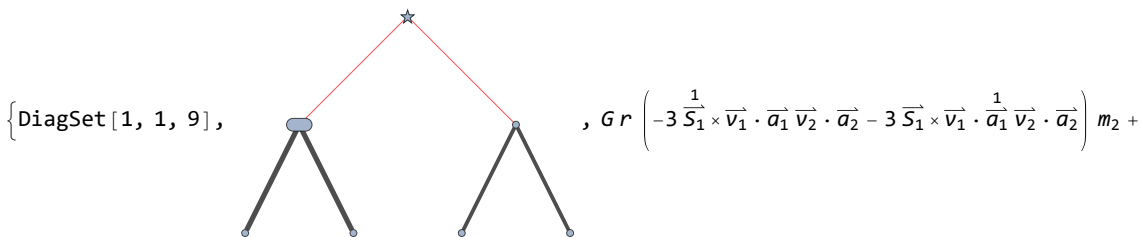

$$G \left( 3 \vec{S_1} \times \vec{v_1} \cdot \vec{a_1} \hat{n} \cdot \vec{v_2} \vec{v_1} \cdot \vec{a_1} + 3 \hat{n} \times \vec{S_1} \cdot \vec{v_1} \vec{v_2} \cdot \vec{a_2} \vec{v_1} \cdot \vec{a_1} + \frac{3}{2} \vec{S_1} \times \vec{v_1} \cdot \vec{a_1} \hat{n} \cdot \vec{v_2} \vec{v_1} \cdot \vec{v_1} + \frac{3}{2} \vec{S_1} \times \vec{v_1} \cdot \vec{a_1} \hat{n} \cdot \vec{v_2} \vec{v_1} \cdot \vec{v_1} - \right. \\ \left. 3 \vec{S_1} \times \vec{v_1} \cdot \vec{a_1} \hat{n} \cdot \vec{v_1} \vec{v_2} \cdot \vec{a_2} + \frac{3}{2} \hat{n} \times \vec{S_1} \cdot \vec{v_1} \vec{v_1} \cdot \vec{v_1} \vec{v_2} \cdot \vec{a_2} + \frac{3}{2} \hat{n} \times \vec{S_1} \cdot \vec{a_1} \vec{v_1} \cdot \vec{v_1} \vec{v_2} \cdot \vec{a_2} + \frac{3}{2} \vec{S_1} \times \vec{v_1} \cdot \vec{a_1} \hat{n} \cdot \vec{v_2} \vec{v_2} \cdot \vec{v_2} + \right. \\ \left. \frac{3}{2} \vec{S_1} \times \vec{v_1} \cdot \vec{a_1} \hat{n} \cdot \vec{v_2} \vec{v_2} \cdot \vec{v_2} + \frac{7}{2} \hat{n} \times \vec{S_1} \cdot \vec{v_1} \vec{v_2} \cdot \vec{a_2} \vec{v_2} \cdot \vec{v_2} + \frac{7}{2} \hat{n} \times \vec{S_1} \cdot \vec{a_1} \vec{v_2} \cdot \vec{a_2} \vec{v_2} \cdot \vec{v_2} \right) m_2 + \frac{1}{r} \\ G \left( -\frac{3}{8} \vec{S_1} \times \vec{v_1} \cdot \vec{v_2} (\vec{v_1} \cdot \vec{v_1})^2 - \frac{3}{8} \vec{S_1} \times \vec{a_1} \cdot \vec{v_2} (\vec{v_1} \cdot \vec{v_1})^2 + \frac{3}{8} \hat{n} \times \vec{S_1} \cdot \vec{v_1} \hat{n} \cdot \vec{v_2} (\vec{v_1} \cdot \vec{v_1})^2 + \frac{3}{8} \hat{n} \times \vec{S_1} \cdot \vec{a_1} \hat{n} \cdot \vec{v_2} (\vec{v_1} \cdot \vec{v_1})^2 - \right.$$

$$\begin{aligned} & \frac{3}{2} \vec{S}_1 \times \vec{v}_1 \cdot \vec{a}_1 \hat{n} \cdot \vec{v}_1 \hat{n} \cdot \vec{v}_2 \vec{v}_1 \cdot \vec{v}_1 - \frac{3}{2} \vec{S}_1 \times \vec{v}_1 \cdot \vec{v}_2 \vec{v}_1 \cdot \vec{a}_1 \vec{v}_1 \cdot \vec{v}_1 + \frac{3}{2} \hat{n} \times \vec{S}_1 \cdot \vec{v}_1 \hat{n} \cdot \vec{v}_2 \vec{v}_1 \cdot \vec{a}_1 \vec{v}_1 \cdot \vec{v}_1 + \\ & \frac{3}{2} \vec{S}_1 \times \vec{v}_1 \cdot \vec{a}_1 \vec{v}_1 \cdot \vec{v}_2 \vec{v}_1 \cdot \vec{v}_1 - \frac{3}{2} \hat{n} \times \vec{S}_1 \cdot \vec{v}_1 \hat{n} \cdot \vec{v}_1 \vec{v}_2 \cdot \vec{a}_2 \vec{v}_1 \cdot \vec{v}_1 - \frac{3}{4} \vec{S}_1 \times \vec{v}_1 \cdot \vec{v}_2 \vec{v}_2 \cdot \vec{v}_2 \vec{v}_1 \cdot \vec{v}_1 - \\ & \frac{3}{4} \vec{S}_1 \times \vec{a}_1 \cdot \vec{v}_2 \vec{v}_2 \cdot \vec{v}_2 \vec{v}_1 \cdot \vec{v}_1 + \frac{3}{4} \hat{n} \times \vec{S}_1 \cdot \vec{v}_1 \hat{n} \cdot \vec{v}_2 \vec{v}_2 \cdot \vec{v}_2 \vec{v}_1 \cdot \vec{v}_1 + \frac{3}{4} \hat{n} \times \vec{S}_1 \cdot \vec{a}_1 \hat{n} \cdot \vec{v}_2 \vec{v}_2 \cdot \vec{v}_2 \vec{v}_1 \cdot \vec{v}_1 - \\ & \frac{7}{8} \vec{S}_1 \times \vec{v}_1 \cdot \vec{v}_2 (\vec{v}_2 \cdot \vec{v}_2)^2 - \frac{7}{8} \vec{S}_1 \times \vec{a}_1 \cdot \vec{v}_2 (\vec{v}_2 \cdot \vec{v}_2)^2 + \frac{7}{8} \hat{n} \times \vec{S}_1 \cdot \vec{v}_1 \hat{n} \cdot \vec{v}_2 (\vec{v}_2 \cdot \vec{v}_2)^2 + \\ & \frac{7}{8} \hat{n} \times \vec{S}_1 \cdot \vec{a}_1 \hat{n} \cdot \vec{v}_2 (\vec{v}_2 \cdot \vec{v}_2)^2 - \frac{3}{2} \vec{S}_1 \times \vec{v}_1 \cdot \vec{a}_1 \hat{n} \cdot \vec{v}_1 \hat{n} \cdot \vec{v}_2 \vec{v}_2 \cdot \vec{v}_2 - \frac{3}{2} \vec{S}_1 \times \vec{v}_1 \cdot \vec{v}_2 \vec{v}_1 \cdot \vec{a}_1 \vec{v}_2 \cdot \vec{v}_2 + \\ & \frac{3}{2} \hat{n} \times \vec{S}_1 \cdot \vec{v}_1 \hat{n} \cdot \vec{v}_2 \vec{v}_1 \cdot \vec{a}_1 \vec{v}_2 \cdot \vec{v}_2 + \frac{3}{2} \vec{S}_1 \times \vec{v}_1 \cdot \vec{a}_1 \vec{v}_1 \cdot \vec{v}_2 \vec{v}_2 \cdot \vec{v}_2 - \frac{7}{2} \hat{n} \times \vec{S}_1 \cdot \vec{v}_1 \hat{n} \cdot \vec{v}_1 \vec{v}_2 \cdot \vec{a}_2 \vec{v}_2 \cdot \vec{v}_2 \Big) m_2 + \\ & \frac{1}{n^2} G \left( \frac{3}{8} \vec{S}_1 \times \vec{v}_1 \cdot \vec{v}_2 \hat{n} \cdot \vec{v}_1 (\vec{v}_1 \cdot \vec{v}_1)^2 - \frac{9}{8} \hat{n} \times \vec{S}_1 \cdot \vec{v}_1 \hat{n} \cdot \vec{v}_1 \hat{n} \cdot \vec{v}_2 (\vec{v}_1 \cdot \vec{v}_1)^2 + \frac{3}{8} \hat{n} \times \vec{S}_1 \cdot \vec{v}_1 \vec{v}_1 \cdot \vec{v}_2 (\vec{v}_1 \cdot \vec{v}_1)^2 + \right. \\ & \frac{3}{4} \vec{S}_1 \times \vec{v}_1 \cdot \vec{v}_2 \hat{n} \cdot \vec{v}_1 \vec{v}_2 \cdot \vec{v}_2 \vec{v}_1 \cdot \vec{v}_1 - \frac{9}{4} \hat{n} \times \vec{S}_1 \cdot \vec{v}_1 \hat{n} \cdot \vec{v}_1 \hat{n} \cdot \vec{v}_2 \vec{v}_2 \cdot \vec{v}_2 \vec{v}_1 \cdot \vec{v}_1 + \frac{3}{4} \hat{n} \times \vec{S}_1 \cdot \vec{v}_1 \vec{v}_1 \cdot \vec{v}_2 \vec{v}_2 \cdot \vec{v}_2 \vec{v}_1 \cdot \vec{v}_1 + \\ & \left. \frac{7}{8} \vec{S}_1 \times \vec{v}_1 \cdot \vec{v}_2 \hat{n} \cdot \vec{v}_1 (\vec{v}_2 \cdot \vec{v}_2)^2 - \frac{21}{8} \hat{n} \times \vec{S}_1 \cdot \vec{v}_1 \hat{n} \cdot \vec{v}_1 \hat{n} \cdot \vec{v}_2 (\vec{v}_2 \cdot \vec{v}_2)^2 + \frac{7}{8} \hat{n} \times \vec{S}_1 \cdot \vec{v}_1 \vec{v}_1 \cdot \vec{v}_2 (\vec{v}_2 \cdot \vec{v}_2)^2 \right) m_2 \Big\} \end{aligned}$$

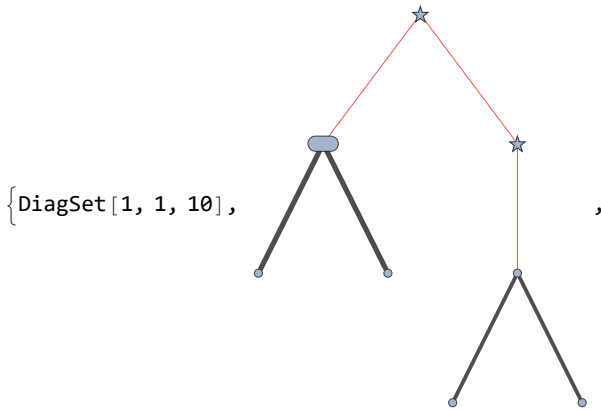

$$\begin{aligned}
G & \left( -\frac{1}{2} \frac{1}{S_1} \times \vec{v}_1 \cdot \frac{1}{a_1} \hat{n} \cdot \vec{a}_2 - \frac{1}{4} \frac{1}{S_1} \times \vec{v}_1 \cdot \vec{a}_1 \hat{n} \cdot \vec{a}_2 - \frac{1}{4} \frac{1}{S_1} \times \vec{a}_1 \cdot \frac{1}{a_1} \hat{n} \cdot \vec{a}_2 - \frac{1}{4} \frac{1}{S_1} \times \vec{v}_1 \cdot \frac{2}{a_1} \hat{n} \cdot \vec{a}_2 - \frac{3}{2} \hat{n} \times \frac{1}{S_1} \cdot \vec{a}_1 \vec{a}_2 \cdot \vec{a}_2 - \right. \\
& \left. \frac{3}{4} \hat{n} \times \frac{1}{S_1} \cdot \vec{v}_1 \vec{a}_2 \cdot \vec{a}_2 - \frac{3}{4} \hat{n} \times \vec{S}_1 \cdot \frac{1}{a_1} \vec{a}_2 \cdot \vec{a}_2 - \frac{3}{2} \hat{n} \times \frac{1}{S_1} \cdot \vec{a}_1 \vec{v}_2 \cdot \vec{a}_2 - \frac{3}{4} \hat{n} \times \frac{2}{S_1} \cdot \vec{v}_1 \vec{v}_2 \cdot \vec{a}_2 - \frac{3}{4} \hat{n} \times \vec{S}_1 \cdot \frac{1}{a_1} \vec{v}_2 \cdot \vec{a}_2 \right) m_2 r^2 + \\
G & \left( \frac{1}{2} \frac{1}{S_1} \times \vec{v}_1 \cdot \frac{1}{a_1} (\hat{n} \cdot \vec{v}_2)^2 + \frac{1}{4} \frac{2}{S_1} \times \vec{v}_1 \cdot \vec{a}_1 (\hat{n} \cdot \vec{v}_2)^2 + \frac{1}{4} \vec{S}_1 \times \vec{a}_1 \cdot \frac{1}{a_1} (\hat{n} \cdot \vec{v}_2)^2 + \frac{1}{4} \vec{S}_1 \times \vec{v}_1 \cdot \frac{2}{a_1} (\hat{n} \cdot \vec{v}_2)^2 + \right. \\
& 3 \hat{n} \times \frac{1}{S_1} \cdot \vec{a}_1 \vec{v}_2 \cdot \vec{a}_2 \hat{n} \cdot \vec{v}_2 + \frac{3}{2} \hat{n} \times \frac{2}{S_1} \cdot \vec{v}_1 \vec{v}_2 \cdot \vec{a}_2 \hat{n} \cdot \vec{v}_2 + \frac{3}{2} \hat{n} \times \vec{S}_1 \cdot \frac{1}{a_1} \vec{v}_2 \cdot \vec{a}_2 \hat{n} \cdot \vec{v}_2 - \frac{1}{4} \vec{S}_1 \times \vec{v}_1 \cdot \vec{a}_1 \hat{n} \cdot \vec{a}_1 \hat{n} \cdot \vec{a}_2 - \\
& \frac{1}{2} \frac{1}{S_1} \times \vec{v}_1 \cdot \vec{a}_1 \hat{n} \cdot \vec{a}_2 \hat{n} \cdot \vec{v}_1 - \frac{1}{2} \vec{S}_1 \times \vec{v}_1 \cdot \frac{1}{a_1} \hat{n} \cdot \vec{a}_2 \hat{n} \cdot \vec{v}_1 + \frac{1}{4} \vec{S}_1 \times \vec{v}_1 \cdot \vec{a}_2 \vec{a}_1 \cdot \vec{a}_1 + \frac{1}{4} \hat{n} \times \vec{S}_1 \cdot \vec{v}_1 \hat{n} \cdot \vec{a}_2 \vec{a}_1 \cdot \vec{a}_1 - \\
& \frac{1}{4} \vec{S}_1 \times \vec{v}_1 \cdot \vec{a}_1 \vec{a}_1 \cdot \vec{a}_2 + \frac{3}{4} \vec{S}_1 \times \vec{v}_1 \cdot \vec{a}_1 \vec{a}_2 \cdot \vec{a}_2 - \frac{3}{4} \hat{n} \times \vec{S}_1 \cdot \vec{v}_1 \hat{n} \cdot \vec{a}_1 \vec{a}_2 \cdot \vec{a}_2 - \frac{3}{2} \hat{n} \times \frac{1}{S_1} \cdot \vec{v}_1 \hat{n} \cdot \vec{v}_1 \vec{a}_2 \cdot \vec{a}_2 - \\
& \frac{3}{2} \hat{n} \times \vec{S}_1 \cdot \vec{a}_1 \hat{n} \cdot \vec{v}_1 \vec{a}_2 \cdot \vec{a}_2 + \frac{1}{4} \vec{S}_1 \times \vec{v}_1 \cdot \vec{a}_2 \vec{v}_1 \cdot \vec{a}_1 + \frac{1}{4} \hat{n} \times \vec{S}_1 \cdot \vec{v}_1 \hat{n} \cdot \vec{a}_2 \vec{v}_1 \cdot \vec{a}_1 + \frac{1}{2} \frac{1}{S_1} \times \vec{v}_1 \cdot \vec{a}_2 \vec{v}_1 \cdot \vec{a}_1 + \\
& \frac{1}{2} \vec{S}_1 \times \vec{a}_1 \cdot \vec{a}_2 \vec{v}_1 \cdot \vec{a}_1 + \frac{1}{2} \hat{n} \times \frac{1}{S_1} \cdot \vec{v}_1 \hat{n} \cdot \vec{a}_2 \vec{v}_1 \cdot \vec{a}_1 + \frac{1}{2} \hat{n} \times \vec{S}_1 \cdot \vec{a}_1 \hat{n} \cdot \vec{a}_2 \vec{v}_1 \cdot \vec{a}_1 - \frac{1}{2} \frac{1}{S_1} \times \vec{v}_1 \cdot \vec{a}_1 \vec{v}_1 \cdot \vec{a}_2 - \\
& \frac{1}{2} \vec{S}_1 \times \vec{v}_1 \cdot \frac{1}{a_1} \vec{v}_1 \cdot \vec{a}_2 + \frac{1}{4} \vec{S}_1 \times \vec{a}_1 \cdot \vec{a}_2 \vec{v}_1 \cdot \vec{v}_1 + \frac{1}{8} \frac{2}{S_1} \times \vec{v}_1 \cdot \vec{a}_2 \vec{v}_1 \cdot \vec{v}_1 + \frac{1}{8} \vec{S}_1 \times \vec{a}_1 \cdot \vec{a}_2 \vec{v}_1 \cdot \vec{v}_1 + \\
& \frac{1}{4} \hat{n} \times \frac{1}{S_1} \cdot \vec{a}_1 \hat{n} \cdot \vec{a}_2 \vec{v}_1 \cdot \vec{v}_1 + \frac{1}{8} \hat{n} \times \frac{2}{S_1} \cdot \vec{v}_1 \hat{n} \cdot \vec{a}_2 \vec{v}_1 \cdot \vec{v}_1 + \frac{1}{8} \hat{n} \times \vec{S}_1 \cdot \frac{1}{a_1} \hat{n} \cdot \vec{a}_2 \vec{v}_1 \cdot \vec{v}_1 + \frac{3}{4} \vec{S}_1 \times \vec{v}_1 \cdot \vec{a}_1 \vec{v}_2 \cdot \vec{a}_2 -
\end{aligned}$$

*G*

[illegible]

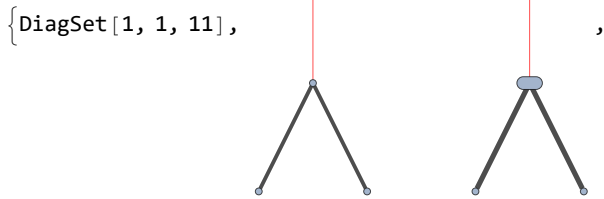

[illegible]

[illegible]





$$\begin{aligned}
 & \frac{3}{8} \vec{S}_1 \times \vec{v}_1 \cdot \vec{v}_2 \hat{n} \cdot \vec{a}_1 \vec{v}_2 \cdot \vec{v}_2 \hat{n} \cdot \vec{v}_1 - \frac{3}{8} \vec{S}_1 \times \vec{v}_1 \cdot \vec{a}_1 \hat{n} \cdot \vec{v}_2 \vec{v}_2 \cdot \vec{v}_2 \hat{n} \cdot \vec{v}_1 - \frac{9}{8} \hat{n} \times \vec{S}_1 \cdot \vec{v}_1 \hat{n} \cdot \vec{a}_1 \hat{n} \cdot \vec{v}_2 \vec{v}_2 \cdot \vec{v}_2 \hat{n} \cdot \vec{v}_1 + \\
 & \frac{3}{8} \hat{n} \times \vec{S}_1 \cdot \vec{v}_1 \vec{a}_1 \cdot \vec{v}_2 \vec{v}_2 \cdot \vec{v}_2 \hat{n} \cdot \vec{v}_1 + \frac{3}{4} \hat{n} \times \vec{S}_1 \cdot \vec{v}_1 \vec{v}_1 \cdot \vec{v}_2 \vec{v}_2 \cdot \vec{v}_2 \hat{n} \cdot \vec{v}_1 + \frac{3}{4} \hat{n} \times \vec{S}_1 \cdot \vec{a}_1 \vec{v}_1 \cdot \vec{v}_2 \vec{v}_2 \cdot \vec{v}_2 \hat{n} \cdot \vec{v}_1 - \\
 & \frac{3}{4} \vec{S}_1 \times \vec{v}_1 \cdot \vec{v}_2 (\vec{v}_1 \cdot \vec{v}_2)^2 - \frac{3}{4} \vec{S}_1 \times \vec{a}_1 \cdot \vec{v}_2 (\vec{v}_1 \cdot \vec{v}_2)^2 + \frac{3}{4} \hat{n} \times \vec{S}_1 \cdot \vec{v}_1 \hat{n} \cdot \vec{v}_2 (\vec{v}_1 \cdot \vec{v}_2)^2 + \\
 & \frac{3}{4} \hat{n} \times \vec{S}_1 \cdot \vec{a}_1 \hat{n} \cdot \vec{v}_2 (\vec{v}_1 \cdot \vec{v}_2)^2 - \frac{3}{8} \hat{n} \times \vec{S}_1 \cdot \vec{v}_1 (\hat{n} \cdot \vec{v}_2)^3 \vec{v}_1 \cdot \vec{a}_1 + \frac{3}{8} \vec{S}_1 \times \vec{v}_1 \cdot \vec{v}_2 (\hat{n} \cdot \vec{v}_2)^2 \vec{v}_1 \cdot \vec{a}_1 - \\
 & \frac{3}{8} \hat{n} \times \vec{S}_1 \cdot \vec{v}_1 (\hat{n} \cdot \vec{v}_2)^3 \vec{v}_1 \cdot \vec{v}_1 - \frac{3}{8} \hat{n} \times \vec{S}_1 \cdot \vec{a}_1 (\hat{n} \cdot \vec{v}_2)^3 \vec{v}_1 \cdot \vec{v}_1 + \frac{3}{8} \vec{S}_1 \times \vec{v}_1 \cdot \vec{v}_2 (\hat{n} \cdot \vec{v}_2)^2 \vec{v}_1 \cdot \vec{v}_1 + \\
 & \frac{3}{8} \vec{S}_1 \times \vec{a}_1 \cdot \vec{v}_2 (\hat{n} \cdot \vec{v}_2)^2 \vec{v}_1 \cdot \vec{v}_1 + \frac{3}{8} \vec{S}_1 \times \vec{v}_1 \cdot \vec{v}_2 \vec{v}_1 \cdot \vec{a}_2 \vec{v}_1 \cdot \vec{v}_1 - \frac{3}{8} \hat{n} \times \vec{S}_1 \cdot \vec{v}_1 \hat{n} \cdot \vec{v}_2 \vec{v}_1 \cdot \vec{a}_2 \vec{v}_1 \cdot \vec{v}_1 - \\
 & \frac{3}{8} \vec{S}_1 \times \vec{v}_1 \cdot \vec{a}_1 (\hat{n} \cdot \vec{v}_2)^2 \vec{v}_1 \cdot \vec{v}_2 - \frac{9}{8} \hat{n} \times \vec{S}_1 \cdot \vec{v}_1 \hat{n} \cdot \vec{a}_1 (\hat{n} \cdot \vec{v}_2)^2 \vec{v}_1 \cdot \vec{v}_2 + \frac{3}{4} \vec{S}_1 \times \vec{v}_1 \cdot \vec{v}_2 \hat{n} \cdot \vec{a}_1 \hat{n} \cdot \vec{v}_2 \vec{v}_1 \cdot \vec{v}_2 - \\
 & \frac{3}{4} \vec{S}_1 \times \vec{v}_1 \cdot \vec{v}_2 \vec{a}_1 \cdot \vec{v}_2 \vec{v}_1 \cdot \vec{v}_2 + \frac{3}{4} \hat{n} \times \vec{S}_1 \cdot \vec{v}_1 \hat{n} \cdot \vec{v}_2 \vec{a}_1 \cdot \vec{v}_2 \vec{v}_1 \cdot \vec{v}_2 + \frac{3}{8} \vec{S}_1 \times \vec{v}_1 \cdot \vec{a}_2 \vec{v}_1 \cdot \vec{v}_1 \vec{v}_1 \cdot \vec{v}_2 - \\
 & \frac{3}{8} \hat{n} \times \vec{S}_1 \cdot \vec{v}_1 \hat{n} \cdot \vec{a}_2 \vec{v}_1 \cdot \vec{v}_1 \vec{v}_1 \cdot \vec{v}_2 - \frac{3}{8} \vec{S}_1 \times \vec{v}_1 \cdot \vec{v}_2 \vec{v}_1 \cdot \vec{a}_1 \vec{v}_2 \cdot \vec{v}_2 + \frac{3}{8} \hat{n} \times \vec{S}_1 \cdot \vec{v}_1 \hat{n} \cdot \vec{v}_2 \vec{v}_1 \cdot \vec{a}_1 \vec{v}_2 \cdot \vec{v}_2 - \\
 & \frac{3}{8} \vec{S}_1 \times \vec{v}_1 \cdot \vec{v}_2 \vec{v}_1 \cdot \vec{v}_1 \vec{v}_2 \cdot \vec{v}_2 - \frac{3}{8} \vec{S}_1 \times \vec{a}_1 \cdot \vec{v}_2 \vec{v}_1 \cdot \vec{v}_1 \vec{v}_2 \cdot \vec{v}_2 + \frac{3}{8} \hat{n} \times \vec{S}_1 \cdot \vec{v}_1 \hat{n} \cdot \vec{v}_2 \vec{v}_1 \cdot \vec{v}_1 \vec{v}_2 \cdot \vec{v}_2 + \\
 & \frac{3}{8} \hat{n} \times \vec{S}_1 \cdot \vec{a}_1 \hat{n} \cdot \vec{v}_2 \vec{v}_1 \cdot \vec{v}_1 \vec{v}_2 \cdot \vec{v}_2 + \frac{3}{8} \vec{S}_1 \times \vec{v}_1 \cdot \vec{a}_1 \vec{v}_1 \cdot \vec{v}_2 \vec{v}_2 \cdot \vec{v}_2 + \frac{3}{8} \hat{n} \times \vec{S}_1 \cdot \vec{v}_1 \hat{n} \cdot \vec{a}_1 \vec{v}_1 \cdot \vec{v}_2 \vec{v}_2 \cdot \vec{v}_2 \Big) m_2 + \frac{1}{\rho^2} \\
 G \Big( & -\frac{35}{8} \hat{n} \times \vec{S}_1 \cdot \vec{v}_1 (\hat{n} \cdot \vec{v}_2)^3 (\hat{n} \cdot \vec{v}_1)^3 + \frac{15}{8} \vec{S}_1 \times \vec{v}_1 \cdot \vec{v}_2 (\hat{n} \cdot \vec{v}_2)^2 (\hat{n} \cdot \vec{v}_1)^3 - \frac{3}{8} \vec{S}_1 \times \vec{v}_1 \cdot \vec{v}_2 \vec{v}_2 \cdot \vec{v}_2 (\hat{n} \cdot \vec{v}_1)^3 + \\
 & \frac{15}{8} \hat{n} \times \vec{S}_1 \cdot \vec{v}_1 \hat{n} \cdot \vec{v}_2 \vec{v}_2 \cdot \vec{v}_2 (\hat{n} \cdot \vec{v}_1)^3 + \frac{45}{8} \hat{n} \times \vec{S}_1 \cdot \vec{v}_1 (\hat{n} \cdot \vec{v}_2)^2 \vec{v}_1 \cdot \vec{v}_2 (\hat{n} \cdot \vec{v}_1)^2 - \\
 & \frac{9}{4} \vec{S}_1 \times \vec{v}_1 \cdot \vec{v}_2 \hat{n} \cdot \vec{v}_2 \vec{v}_1 \cdot \vec{v}_2 (\hat{n} \cdot \vec{v}_1)^2 - \frac{9}{8} \hat{n} \times \vec{S}_1 \cdot \vec{v}_1 \vec{v}_1 \cdot \vec{v}_2 \vec{v}_2 \cdot \vec{v}_2 (\hat{n} \cdot \vec{v}_1)^2 + \frac{3}{4} \vec{S}_1 \times \vec{v}_1 \cdot \vec{v}_2 (\vec{v}_1 \cdot \vec{v}_2)^2 \hat{n} \cdot \vec{v}_1 - \\
 & \frac{9}{4} \hat{n} \times \vec{S}_1 \cdot \vec{v}_1 \hat{n} \cdot \vec{v}_2 (\vec{v}_1 \cdot \vec{v}_2)^2 \hat{n} \cdot \vec{v}_1 + \frac{15}{8} \hat{n} \times \vec{S}_1 \cdot \vec{v}_1 (\hat{n} \cdot \vec{v}_2)^3 \vec{v}_1 \cdot \vec{v}_1 \hat{n} \cdot \vec{v}_1 - \frac{9}{8} \vec{S}_1 \times \vec{v}_1 \cdot \vec{v}_2 (\hat{n} \cdot \vec{v}_2)^2 \vec{v}_1 \cdot \vec{v}_1 \hat{n} \cdot \vec{v}_1 + \\
 & \frac{3}{8} \vec{S}_1 \times \vec{v}_1 \cdot \vec{v}_2 \vec{v}_1 \cdot \vec{v}_1 \vec{v}_2 \cdot \vec{v}_2 \hat{n} \cdot \vec{v}_1 - \frac{9}{8} \hat{n} \times \vec{S}_1 \cdot \vec{v}_1 \hat{n} \cdot \vec{v}_2 \vec{v}_1 \cdot \vec{v}_1 \vec{v}_2 \cdot \vec{v}_2 \hat{n} \cdot \vec{v}_1 + \frac{1}{4} \hat{n} \times \vec{S}_1 \cdot \vec{v}_1 (\vec{v}_1 \cdot \vec{v}_2)^3 - \\
 & \frac{9}{8} \hat{n} \times \vec{S}_1 \cdot \vec{v}_1 (\hat{n} \cdot \vec{v}_2)^2 \vec{v}_1 \cdot \vec{v}_1 \vec{v}_1 \cdot \vec{v}_2 + \frac{3}{4} \vec{S}_1 \times \vec{v}_1 \cdot \vec{v}_2 \hat{n} \cdot \vec{v}_2 \vec{v}_1 \cdot \vec{v}_1 \vec{v}_1 \cdot \vec{v}_2 + \frac{3}{8} \hat{n} \times \vec{S}_1 \cdot \vec{v}_1 \vec{v}_1 \cdot \vec{v}_1 \vec{v}_1 \cdot \vec{v}_2 \vec{v}_2 \cdot \vec{v}_2 \Big) m_2 \Big\}
 \end{aligned}$$

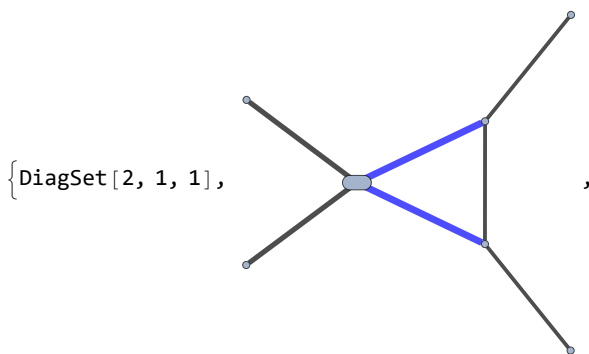

$$\frac{2 G^2 m_2^2 \vec{v}_2 \cdot \vec{v}_2 \vec{S}_1 \times \vec{v}_2 \cdot \vec{a}_2}{\rho^2} + \frac{1}{\rho^3} G^2 m_2^2 \left( -8 (\vec{v}_2 \cdot \vec{v}_2)^2 \hat{n} \times \vec{S}_1 \cdot \vec{v}_1 + 4 \vec{v}_2 \cdot \vec{v}_2 \hat{n} \cdot \vec{v}_2 \vec{S}_1 \times \vec{v}_1 \cdot \vec{v}_2 + 8 \vec{v}_1 \cdot \vec{v}_2 \vec{v}_2 \cdot \vec{v}_2 \hat{n} \times \vec{S}_1 \cdot \vec{v}_2 \right) \Big\}$$

$\{\text{DiagSet}[2, 1, 2],$ 
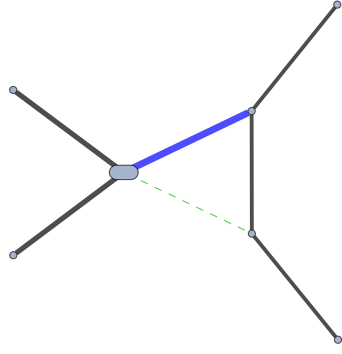

$$, \frac{G^2 m_2^2 \left( -16 \vec{v}_1 \cdot \vec{v}_2 \vec{S}_1 \times \vec{v}_2 \cdot \vec{a}_2 - 8 \vec{v}_2 \cdot \vec{a}_2 \vec{S}_1 \times \vec{v}_1 \cdot \vec{v}_2 \right)}{r^2} + \frac{1}{r^3}$$

$$G^2 m_2^2 \left( -6 (\vec{v}_1 \cdot \vec{v}_2)^2 \hat{n} \times \vec{S}_1 \cdot \vec{v}_2 + 6 \vec{v}_1 \cdot \vec{v}_2 \hat{n} \cdot \vec{v}_2 \vec{S}_1 \times \vec{v}_1 \cdot \vec{v}_2 - 4 (\vec{v}_2 \cdot \vec{v}_2)^2 \hat{n} \times \vec{S}_1 \cdot \vec{v}_2 - 6 \vec{v}_2 \cdot \vec{v}_2 \hat{n} \cdot \vec{v}_1 \vec{S}_1 \times \vec{v}_1 \cdot \vec{v}_2 \right) \}$$

 $\{\text{DiagSet}[2, 1, 3],$ 
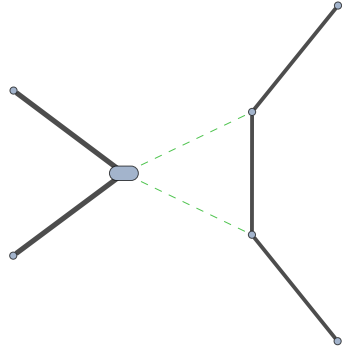
 $,$ 

$$\frac{G^2 m_2^2 \left( -12 \vec{v}_1 \cdot \vec{a}_2 \vec{S}_1 \times \vec{v}_1 \cdot \vec{v}_2 + 12 \vec{v}_1 \cdot \vec{v}_2 \vec{S}_1 \times \vec{v}_1 \cdot \vec{a}_2 + 8 \vec{v}_2 \cdot \vec{v}_2 \vec{S}_1 \times \vec{v}_2 \cdot \vec{a}_2 \right)}{r^2} + \frac{1}{r^3}$$

$$G^2 m_2^2 \left( 12 (\vec{v}_1 \cdot \vec{v}_2)^2 \hat{n} \times \vec{S}_1 \cdot \vec{v}_1 - 12 \vec{v}_1 \cdot \vec{v}_2 \hat{n} \cdot \vec{v}_1 \vec{S}_1 \times \vec{v}_1 \cdot \vec{v}_2 - 8 \vec{v}_2 \cdot \vec{v}_2 \vec{v}_1 \cdot \vec{v}_2 \hat{n} \times \vec{S}_1 \cdot \vec{v}_2 \right) \}$$

 $\{\text{DiagSet}[2, 1, 4],$ 
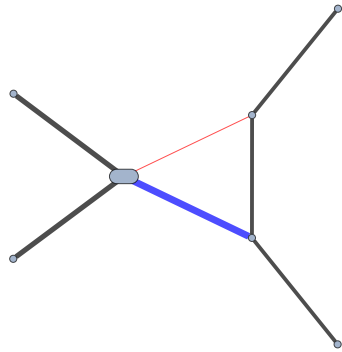
 $,$ 

$$\frac{1}{r^2} G^2 m_2^2 \left( 4 \vec{a}_1 \cdot \vec{v}_2 \vec{S}_1 \times \vec{v}_1 \cdot \vec{v}_2 + 12 \vec{v}_1 \cdot \vec{a}_2 \vec{S}_1 \times \vec{v}_1 \cdot \vec{v}_2 - 4 \vec{v}_1 \cdot \vec{v}_2 \vec{S}_1 \times \vec{a}_1 \cdot \vec{v}_2 + 12 \vec{v}_1 \cdot \vec{v}_2 \vec{S}_1 \times \vec{v}_1 \cdot \vec{a}_2 - 8 \vec{v}_2 \cdot \vec{v}_2 \vec{S}_1 \times \vec{v}_1 \cdot \vec{a}_1 \right) +$$

$$\frac{1}{r^3} G^2 m_2^2 \left( 8 (\vec{v}_1 \cdot \vec{v}_2)^2 \hat{n} \times \vec{S}_1 \cdot \vec{v}_1 - 8 \vec{v}_1 \cdot \vec{v}_2 \hat{n} \cdot \vec{v}_1 \vec{S}_1 \times \vec{v}_1 \cdot \vec{v}_2 + 12 \vec{v}_1 \cdot \vec{v}_2 \hat{n} \cdot \vec{v}_2 \vec{S}_1 \times \vec{v}_1 \cdot \vec{v}_2 + 2 \vec{v}_1 \cdot \vec{v}_1 \vec{v}_1 \cdot \vec{v}_2 \hat{n} \times \vec{S}_1 \cdot \vec{v}_2 + \right.$$

$$\left. 8 \vec{v}_2 \cdot \vec{v}_2 \vec{v}_1 \cdot \vec{v}_2 \hat{n} \times \vec{S}_1 \cdot \vec{v}_2 - 2 \vec{v}_1 \cdot \vec{v}_1 \hat{n} \cdot \vec{v}_2 \vec{S}_1 \times \vec{v}_1 \cdot \vec{v}_2 - 8 \vec{v}_2 \cdot \vec{v}_2 \hat{n} \cdot \vec{v}_2 \vec{S}_1 \times \vec{v}_1 \cdot \vec{v}_2 - 8 \vec{v}_1 \cdot \vec{v}_1 \vec{v}_2 \cdot \vec{v}_2 \hat{n} \times \vec{S}_1 \cdot \vec{v}_1 \right) \}$$

{DiagSet[2, 1, 5],

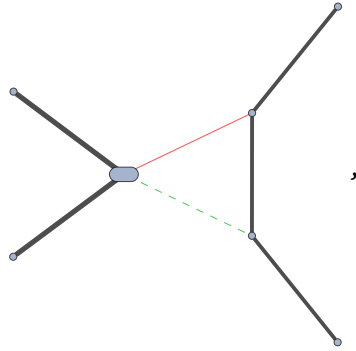

,

$$\frac{G^2 m_2^2 \left( -8 \vec{v}_1 \cdot \vec{v}_1 \vec{S}_1 \times \vec{v}_1 \cdot \vec{a}_2 - 16 \vec{v}_1 \cdot \vec{v}_2 \vec{S}_1 \times \vec{v}_1 \cdot \vec{a}_1 + 24 \vec{v}_2 \cdot \vec{a}_2 \vec{S}_1 \times \vec{v}_1 \cdot \vec{v}_2 \right)}{r^2} +$$

$$\frac{1}{r^3} G^2 m_2^2 \left( 16 (\vec{v}_2 \cdot \vec{v}_2)^2 \hat{n} \times \vec{S}_1 \cdot \vec{v}_2 + 16 \vec{v}_2 \cdot \vec{v}_2 \hat{n} \cdot \vec{v}_2 \vec{S}_1 \times \vec{v}_1 \cdot \vec{v}_2 + \right. \\ \left. 7 \vec{v}_1 \cdot \vec{v}_1 \hat{n} \cdot \vec{v}_1 \vec{S}_1 \times \vec{v}_1 \cdot \vec{v}_2 - 4 \vec{v}_1 \cdot \vec{v}_1 \hat{n} \cdot \vec{v}_2 \vec{S}_1 \times \vec{v}_1 \cdot \vec{v}_2 - 15 \vec{v}_1 \cdot \vec{v}_1 \vec{v}_1 \cdot \vec{v}_2 \hat{n} \times \vec{S}_1 \cdot \vec{v}_1 \right) \Big\}$$

{DiagSet[2, 1, 6],

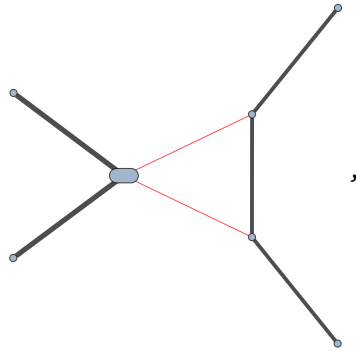

,

$$\frac{G^2 m_2^2 \left( 12 \vec{v}_1 \cdot \vec{v}_1 \vec{S}_1 \times \vec{v}_1 \cdot \vec{a}_1 + 12 \vec{v}_2 \cdot \vec{v}_2 \vec{S}_1 \times \vec{v}_1 \cdot \vec{a}_1 \right)}{r^2} + \frac{G^2 m_2^2 \left( 6 (\vec{v}_1 \cdot \vec{v}_1)^2 \hat{n} \times \vec{S}_1 \cdot \vec{v}_1 + 12 \vec{v}_2 \cdot \vec{v}_2 \vec{v}_1 \cdot \vec{v}_1 \hat{n} \times \vec{S}_1 \cdot \vec{v}_1 \right)}{r^3} \Big\}$$

{DiagSet[2, 1, 7],

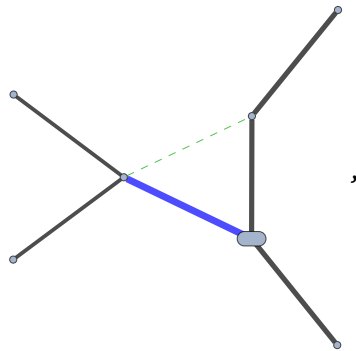

$$\frac{G^2 m_1 m_2 \left( 8 \vec{v}_1 \cdot \vec{v}_2 \vec{v}_2 \cdot \vec{v}_2 \hat{n} \times \vec{S}_1 \cdot \vec{v}_1 - 8 (\vec{v}_1 \cdot \vec{v}_2)^2 \hat{n} \times \vec{S}_1 \cdot \vec{v}_2 \right)}{r^3} \Big\}$$

{DiagSet[2, 1, 8],

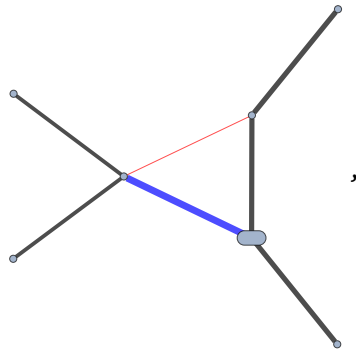

,

$$\frac{1}{r^2} G^2 m_1 m_2 \left( -6 \vec{a}_1 \cdot \vec{v}_2 \vec{S}_1 \times \vec{v}_1 \cdot \vec{v}_2 + 12 \vec{v}_1 \cdot \vec{v}_2 \vec{a}_1 \times \vec{S}_1 \cdot \vec{v}_2 - 6 \vec{v}_2 \cdot \vec{v}_2 \vec{a}_1 \times \vec{S}_1 \cdot \vec{v}_1 - 9 \vec{v}_1 \cdot \vec{v}_2 \vec{S}_1 \times \vec{v}_1 \cdot \vec{v}_2 \right) +$$

$$\frac{1}{r^3} G^2 m_1 m_2 \left( 3 \left( \vec{v}_1 \cdot \vec{v}_2 \right)^2 \hat{n} \times \vec{S}_1 \cdot \vec{v}_1 + 3 \vec{v}_1 \cdot \vec{v}_2 \hat{n} \cdot \vec{v}_1 \vec{S}_1 \times \vec{v}_1 \cdot \vec{v}_2 + 9 \vec{v}_1 \cdot \vec{v}_1 \vec{v}_1 \cdot \vec{v}_2 \hat{n} \times \vec{S}_1 \cdot \vec{v}_2 + \right.$$

$$\left. 7 \vec{v}_2 \cdot \vec{v}_2 \vec{v}_1 \cdot \vec{v}_2 \hat{n} \times \vec{S}_1 \cdot \vec{v}_2 - 7 \left( \vec{v}_2 \cdot \vec{v}_2 \right)^2 \hat{n} \times \vec{S}_1 \cdot \vec{v}_1 - 12 \vec{v}_1 \cdot \vec{v}_1 \vec{v}_2 \cdot \vec{v}_2 \hat{n} \times \vec{S}_1 \cdot \vec{v}_1 \right) \}$$

$\{\text{DiagSet}[2, 1, 9],$

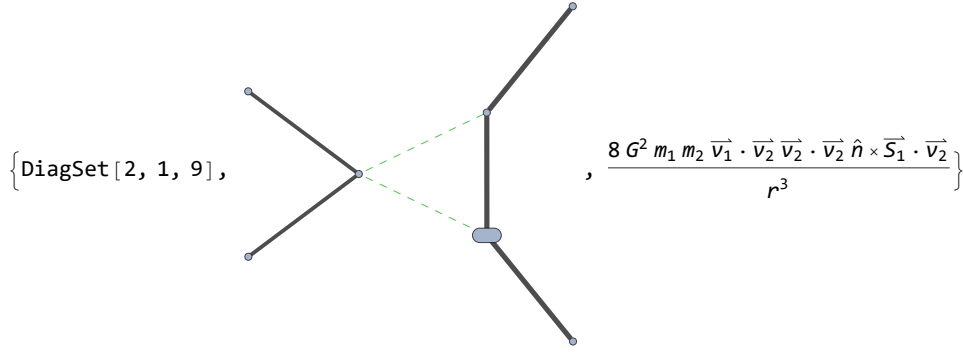

$, \frac{8 G^2 m_1 m_2 \vec{v}_1 \cdot \vec{v}_2 \vec{v}_2 \cdot \vec{v}_2 \hat{n} \times \vec{S}_1 \cdot \vec{v}_2}{r^3} \}$

$\{\text{DiagSet}[2, 1, 10],$

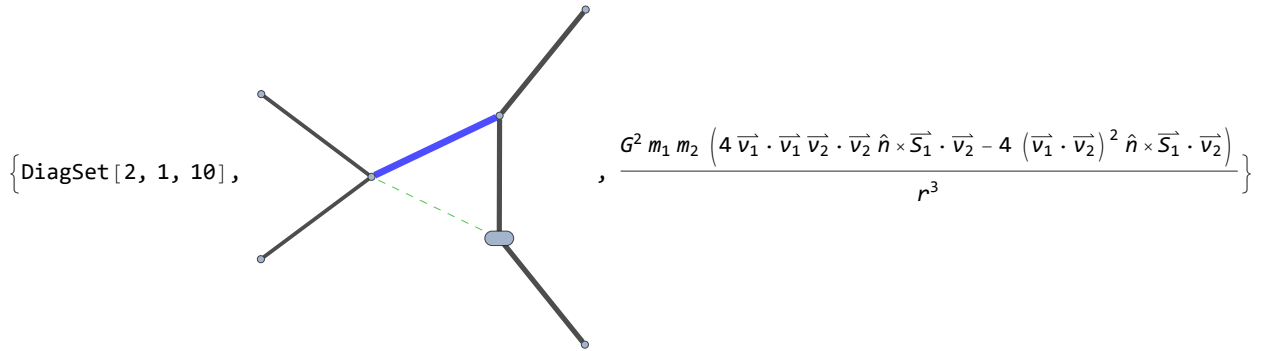

$, \frac{G^2 m_1 m_2 \left( 4 \vec{v}_1 \cdot \vec{v}_1 \vec{v}_2 \cdot \vec{v}_2 \hat{n} \times \vec{S}_1 \cdot \vec{v}_2 - 4 \left( \vec{v}_1 \cdot \vec{v}_2 \right)^2 \hat{n} \times \vec{S}_1 \cdot \vec{v}_2 \right)}{r^3} \}$

$\{\text{DiagSet}[2, 1, 11],$

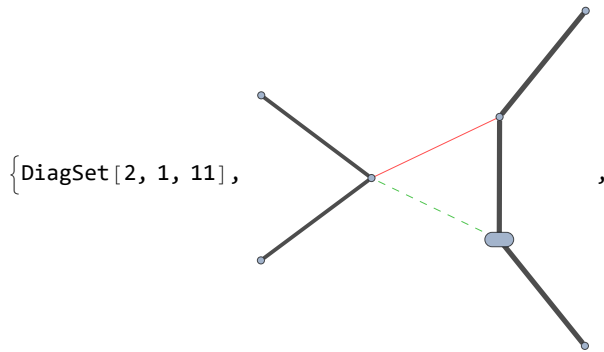

$,$

$$\frac{1}{r^2} G^2 m_1 m_2 \left( -4 \vec{a}_1 \cdot \vec{v}_1 \vec{S}_1 \times \vec{v}_1 \cdot \vec{v}_2 + 8 \vec{v}_1 \cdot \vec{v}_1 \vec{a}_1 \times \vec{S}_1 \cdot \vec{v}_2 + 4 \vec{v}_1 \cdot \vec{v}_2 \vec{a}_1 \times \vec{S}_1 \cdot \vec{v}_1 - \right.$$

$$\left. 6 \vec{v}_2 \cdot \vec{v}_2 \vec{a}_1 \times \vec{S}_1 \cdot \vec{v}_2 - 8 \vec{v}_1 \cdot \vec{v}_1 \vec{S}_1 \times \vec{v}_1 \cdot \vec{v}_2 + 6 \vec{v}_2 \cdot \vec{v}_2 \vec{S}_1 \times \vec{v}_1 \cdot \vec{v}_2 \right) + \frac{1}{r^3}$$

$$G^2 m_1 m_2 \left( \frac{7}{4} \left( \vec{v}_1 \cdot \vec{v}_1 \right)^2 \hat{n} \times \vec{S}_1 \cdot \vec{v}_2 + \frac{7}{4} \vec{v}_1 \cdot \vec{v}_1 \hat{n} \cdot \vec{v}_1 \vec{S}_1 \times \vec{v}_1 \cdot \vec{v}_2 + \frac{25}{4} \vec{v}_1 \cdot \vec{v}_2 \vec{v}_1 \cdot \vec{v}_1 \hat{n} \times \vec{S}_1 \cdot \vec{v}_1 - \right.$$

$$\left. \frac{9}{2} \vec{v}_2 \cdot \vec{v}_2 \vec{v}_1 \cdot \vec{v}_1 \hat{n} \times \vec{S}_1 \cdot \vec{v}_2 - \frac{21}{4} \left( \vec{v}_2 \cdot \vec{v}_2 \right)^2 \hat{n} \times \vec{S}_1 \cdot \vec{v}_2 - \frac{3}{2} \vec{v}_2 \cdot \vec{v}_2 \hat{n} \cdot \vec{v}_1 \vec{S}_1 \times \vec{v}_1 \cdot \vec{v}_2 - \frac{9}{2} \vec{v}_1 \cdot \vec{v}_2 \vec{v}_2 \cdot \vec{v}_2 \hat{n} \times \vec{S}_1 \cdot \vec{v}_1 \right) \}$$

{DiagSet[2, 1, 12],

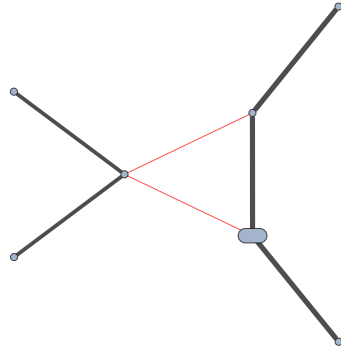

$$, \frac{G^2 m_1 m_2 \left( 9 \vec{v}_2 \cdot \vec{v}_2 \vec{a}_1 \times \vec{S}_1 \cdot \vec{v}_1 - 6 \vec{v}_1 \cdot \vec{v}_1 \vec{a}_1 \times \vec{S}_1 \cdot \vec{v}_1 \right)}{r^2} +$$

$$\frac{1}{r^3} G^2 m_1 m_2 \left( -4 \left( \vec{v}_1 \cdot \vec{v}_1 \right)^2 \hat{n} \times \vec{S}_1 \cdot \vec{v}_1 + 18 \vec{v}_2 \cdot \vec{v}_2 \vec{v}_1 \cdot \vec{v}_1 \hat{n} \times \vec{S}_1 \cdot \vec{v}_1 + \frac{49}{4} \left( \vec{v}_2 \cdot \vec{v}_2 \right)^2 \hat{n} \times \vec{S}_1 \cdot \vec{v}_1 \right) \}$$

{DiagSet[2, 1, 13],

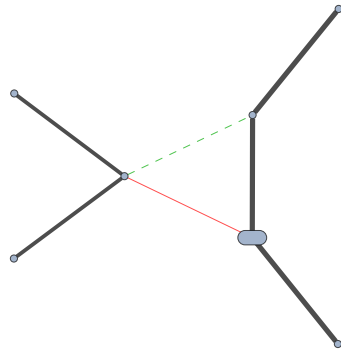

,

$$\frac{8 G^2 m_1 m_2 \vec{v}_1 \cdot \vec{v}_2 \vec{a}_1 \times \vec{S}_1 \cdot \vec{v}_1}{r^2} + \frac{G^2 m_1 m_2 \left( 8 \vec{v}_1 \cdot \vec{v}_1 \vec{v}_1 \cdot \vec{v}_2 \hat{n} \times \vec{S}_1 \cdot \vec{v}_1 - 12 \vec{v}_1 \cdot \vec{v}_2 \vec{v}_2 \cdot \vec{v}_2 \hat{n} \times \vec{S}_1 \cdot \vec{v}_1 \right)}{r^3} \}$$

{DiagSet[2, 1, 14],

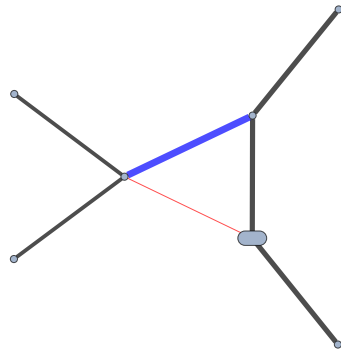

,

$$\frac{G^2 m_1 m_2 \left( 12 \left( \vec{v}_1 \cdot \vec{v}_2 \right)^2 \hat{n} \times \vec{S}_1 \cdot \vec{v}_1 - 12 \vec{v}_1 \cdot \vec{v}_1 \vec{v}_2 \cdot \vec{v}_2 \hat{n} \times \vec{S}_1 \cdot \vec{v}_1 \right)}{r^3} \}$$

{DiagSet[2, 1, 15],

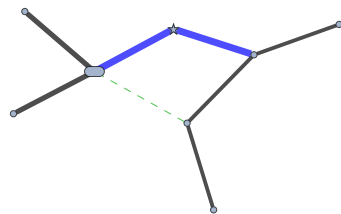

,

$$\frac{1}{r^2} G^2 m_2^2 \left( -8 \left( \hat{n} \cdot \vec{v}_2 \right)^2 \vec{S}_1 \times \vec{v}_2 \cdot \vec{a}_2 + 4 \hat{n} \cdot \vec{v}_1 \hat{n} \cdot \vec{v}_2 \vec{S}_1 \times \vec{v}_2 \cdot \vec{a}_2 + 20 \vec{v}_2 \cdot \vec{a}_2 \hat{n} \cdot \vec{v}_2 \hat{n} \times \vec{S}_1 \cdot \vec{v}_2 - \right. \\ \left. 10 \vec{v}_2 \cdot \vec{v}_2 \hat{n} \cdot \vec{v}_2 \hat{n} \times \vec{S}_1 \cdot \vec{a}_2 - 12 \vec{v}_2 \cdot \vec{a}_2 \hat{n} \cdot \vec{v}_1 \hat{n} \times \vec{S}_1 \cdot \vec{v}_2 + 4 \vec{v}_2 \cdot \vec{v}_2 \hat{n} \cdot \vec{v}_1 \hat{n} \times \vec{S}_1 \cdot \vec{a}_2 - \right.$$

$$\begin{aligned}
& 2 \vec{v}_1 \cdot \vec{v}_2 \vec{S}_1 \times \vec{v}_2 \cdot \vec{a}_2 - 6 \vec{v}_2 \cdot \vec{a}_2 \vec{S}_1 \times \vec{v}_1 \cdot \vec{v}_2 + 2 \vec{v}_2 \cdot \vec{v}_2 \vec{S}_1 \times \vec{v}_1 \cdot \vec{a}_2 - 2 \vec{v}_2 \cdot \vec{v}_2 \hat{n} \cdot \vec{v}_2 \hat{n} \times \vec{S}_1 \cdot \vec{v}_2 \Big) + \\
& \frac{1}{r} G^2 m_2^2 \left( 2 \hat{n} \cdot \vec{a}_2 \vec{S}_1 \times \vec{v}_2 \cdot \vec{a}_2 - 2 \hat{n} \cdot \vec{v}_2 \vec{S}_1 \times \vec{v}_2 \cdot \vec{a}_2 - 2 \vec{a}_2 \cdot \vec{a}_2 \hat{n} \times \vec{S}_1 \cdot \vec{v}_2 + 6 \vec{v}_2 \cdot \vec{a}_2 \hat{n} \times \vec{S}_1 \cdot \vec{v}_2 + \right. \\
& \left. 6 \vec{v}_2 \cdot \vec{a}_2 \hat{n} \times \vec{S}_1 \cdot \vec{a}_2 - 2 \vec{v}_2 \cdot \vec{v}_2 \hat{n} \times \vec{S}_1 \cdot \vec{a}_2 \right) + \frac{1}{r^3} G^2 m_2^2 \left( -6 \vec{v}_2 \cdot \vec{v}_2 (\hat{n} \cdot \vec{v}_2)^2 \hat{n} \times \vec{S}_1 \cdot \vec{v}_2 + \right. \\
& \left. 2 \vec{v}_2 \cdot \vec{v}_2 \hat{n} \cdot \vec{v}_2 \vec{S}_1 \times \vec{v}_1 \cdot \vec{v}_2 + 8 \vec{v}_2 \cdot \vec{v}_2 \hat{n} \cdot \vec{v}_1 \hat{n} \cdot \vec{v}_2 \hat{n} \times \vec{S}_1 \cdot \vec{v}_2 - 2 \vec{v}_1 \cdot \vec{v}_2 \vec{v}_2 \cdot \vec{v}_2 \hat{n} \times \vec{S}_1 \cdot \vec{v}_2 \right) \Big\}
\end{aligned}$$

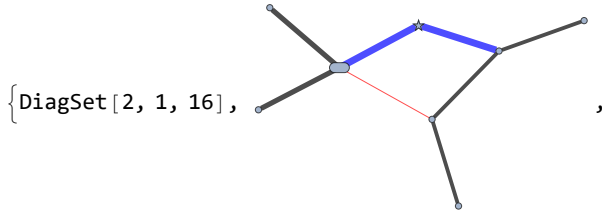

$$\begin{aligned}
& \frac{1}{r} G^2 \left( 2 \vec{S}_1 \times \vec{v}_1 \cdot \vec{v}_2 \hat{n} \cdot \vec{a}_2 + 2 \vec{S}_1 \times \vec{a}_1 \cdot \vec{v}_2 \hat{n} \cdot \vec{a}_2 + 2 \vec{S}_1 \times \vec{v}_1 \cdot \vec{a}_2 \hat{n} \cdot \vec{v}_2 + 2 \vec{S}_1 \times \vec{a}_1 \cdot \vec{a}_2 \hat{n} \cdot \vec{v}_2 - \right. \\
& \left. 2 \hat{n} \times \vec{S}_1 \cdot \vec{v}_2 \vec{a}_1 \cdot \vec{a}_2 - 2 \hat{n} \times \vec{S}_1 \cdot \vec{a}_2 \vec{a}_1 \cdot \vec{v}_2 - 2 \hat{n} \times \vec{S}_1 \cdot \vec{v}_2 \vec{v}_1 \cdot \vec{a}_2 - 2 \hat{n} \times \vec{S}_1 \cdot \vec{a}_2 \vec{v}_1 \cdot \vec{v}_2 \right) m_2^2 + \frac{1}{r^2} \\
& G^2 \left( -2 \vec{S}_1 \times \vec{v}_1 \cdot \vec{v}_2 (\hat{n} \cdot \vec{v}_2)^2 - 2 \vec{S}_1 \times \vec{a}_1 \cdot \vec{v}_2 (\hat{n} \cdot \vec{v}_2)^2 + 6 \vec{S}_1 \times \vec{v}_1 \cdot \vec{a}_2 (\hat{n} \cdot \vec{v}_2)^2 + 6 \vec{S}_1 \times \vec{v}_1 \cdot \vec{v}_2 \hat{n} \cdot \vec{a}_2 \hat{n} \cdot \vec{v}_2 - \right. \\
& 4 \vec{S}_1 \times \vec{v}_1 \cdot \vec{a}_2 \hat{n} \cdot \vec{v}_1 \hat{n} \cdot \vec{v}_2 + 2 \hat{n} \times \vec{S}_1 \cdot \vec{v}_2 \vec{a}_1 \cdot \vec{v}_2 \hat{n} \cdot \vec{v}_2 - 6 \hat{n} \times \vec{S}_1 \cdot \vec{v}_2 \vec{v}_1 \cdot \vec{a}_2 \hat{n} \cdot \vec{v}_2 + 2 \hat{n} \times \vec{S}_1 \cdot \vec{v}_2 \vec{v}_1 \cdot \vec{v}_2 \hat{n} \cdot \vec{v}_2 - \\
& 6 \hat{n} \times \vec{S}_1 \cdot \vec{a}_2 \vec{v}_1 \cdot \vec{v}_2 \hat{n} \cdot \vec{v}_2 - 4 \vec{S}_1 \times \vec{v}_1 \cdot \vec{v}_2 \hat{n} \cdot \vec{a}_2 \hat{n} \cdot \vec{v}_1 + 4 \vec{S}_1 \times \vec{v}_1 \cdot \vec{v}_2 \vec{v}_1 \cdot \vec{a}_2 + 4 \hat{n} \times \vec{S}_1 \cdot \vec{v}_2 \hat{n} \cdot \vec{v}_1 \vec{v}_1 \cdot \vec{a}_2 + \\
& \left. 4 \vec{S}_1 \times \vec{v}_1 \cdot \vec{a}_2 \vec{v}_1 \cdot \vec{v}_2 - 2 \vec{S}_1 \times \vec{v}_2 \cdot \vec{a}_2 \vec{v}_1 \cdot \vec{v}_2 + 4 \hat{n} \times \vec{S}_1 \cdot \vec{a}_2 \hat{n} \cdot \vec{v}_1 \vec{v}_1 \cdot \vec{v}_2 - 2 \vec{S}_1 \times \vec{v}_1 \cdot \vec{v}_2 \vec{v}_2 \cdot \vec{a}_2 - 2 \vec{S}_1 \times \vec{v}_1 \cdot \vec{a}_2 \vec{v}_2 \cdot \vec{v}_2 \right) m_2^2 + \\
& \frac{1}{r^3} G^2 \left( -6 \vec{S}_1 \times \vec{v}_1 \cdot \vec{v}_2 (\hat{n} \cdot \vec{v}_2)^3 + 8 \vec{S}_1 \times \vec{v}_1 \cdot \vec{v}_2 \hat{n} \cdot \vec{v}_1 (\hat{n} \cdot \vec{v}_2)^2 + 6 \hat{n} \times \vec{S}_1 \cdot \vec{v}_2 \vec{v}_1 \cdot \vec{v}_2 (\hat{n} \cdot \vec{v}_2)^2 - \right. \\
& \left. 6 \vec{S}_1 \times \vec{v}_1 \cdot \vec{v}_2 \vec{v}_1 \cdot \vec{v}_2 \hat{n} \cdot \vec{v}_2 - 8 \hat{n} \times \vec{S}_1 \cdot \vec{v}_2 \hat{n} \cdot \vec{v}_1 \vec{v}_1 \cdot \vec{v}_2 \hat{n} \cdot \vec{v}_2 + 2 \vec{S}_1 \times \vec{v}_1 \cdot \vec{v}_2 \vec{v}_2 \cdot \vec{v}_2 \hat{n} \cdot \vec{v}_2 + 2 \hat{n} \times \vec{S}_1 \cdot \vec{v}_2 (\vec{v}_1 \cdot \vec{v}_2)^2 \right) m_2^2 \Big\}
\end{aligned}$$

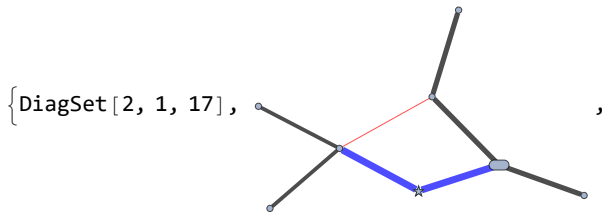

$$\begin{aligned}
& \frac{1}{r} \left( 3 \hat{n} \times \vec{S}_1 \cdot \vec{v}_2 \vec{a}_1 \cdot \vec{a}_2 - 3 \hat{n} \times \vec{a}_2 \cdot \vec{S}_1 \vec{a}_1 \cdot \vec{v}_2 + 3 \hat{n} \times \vec{S}_1 \cdot \vec{v}_2 \vec{a}_2 \cdot \vec{v}_1 - 6 \hat{n} \times \vec{S}_1 \cdot \vec{v}_1 \vec{a}_2 \cdot \vec{v}_2 + \right. \\
& \left. 6 \hat{n} \times \vec{a}_1 \cdot \vec{S}_1 \vec{a}_2 \cdot \vec{v}_2 - 3 \hat{n} \times \vec{a}_2 \cdot \vec{S}_1 \vec{v}_1 \cdot \vec{v}_2 \right) m_1 m_2 G^2 + \frac{1}{r^2} \\
& \left( -3 \hat{n} \times \vec{S}_1 \cdot \vec{v}_2 \hat{n} \cdot \vec{v}_1 \vec{a}_1 \cdot \vec{v}_2 + 6 \hat{n} \times \vec{S}_1 \cdot \vec{v}_2 \hat{n} \cdot \vec{v}_2 \vec{a}_1 \cdot \vec{v}_2 - 3 \vec{S}_1 \times \vec{v}_1 \cdot \vec{v}_2 \vec{a}_2 \cdot \vec{v}_1 - 3 \hat{n} \times \vec{S}_1 \cdot \vec{v}_2 \hat{n} \cdot \vec{v}_1 \vec{a}_2 \cdot \vec{v}_1 + \right. \\
& 6 \hat{n} \times \vec{S}_1 \cdot \vec{v}_1 \hat{n} \cdot \vec{v}_1 \vec{a}_2 \cdot \vec{v}_2 - 3 \vec{a}_2 \times \vec{S}_1 \cdot \vec{v}_1 \vec{v}_1 \cdot \vec{v}_2 - 3 \hat{n} \times \vec{S}_1 \cdot \vec{v}_2 \hat{n} \cdot \vec{v}_1 \vec{v}_1 \cdot \vec{v}_2 + 3 \hat{n} \times \vec{a}_2 \cdot \vec{S}_1 \hat{n} \cdot \vec{v}_1 \vec{v}_1 \cdot \vec{v}_2 + \\
& 6 \hat{n} \times \vec{S}_1 \cdot \vec{v}_2 \hat{n} \cdot \vec{v}_2 \vec{v}_1 \cdot \vec{v}_2 + 3 \vec{S}_1 \times \vec{v}_1 \cdot \vec{v}_2 \vec{v}_2 \cdot \vec{v}_2 - 3 \vec{a}_1 \times \vec{S}_1 \cdot \vec{v}_2 \vec{v}_2 \cdot \vec{v}_2 + 3 \hat{n} \times \vec{S}_1 \cdot \vec{v}_1 \hat{n} \cdot \vec{v}_1 \vec{v}_2 \cdot \vec{v}_2 - \\
& \left. 3 \hat{n} \times \vec{a}_1 \cdot \vec{S}_1 \hat{n} \cdot \vec{v}_1 \vec{v}_2 \cdot \vec{v}_2 - 6 \hat{n} \times \vec{S}_1 \cdot \vec{v}_1 \hat{n} \cdot \vec{v}_2 \vec{v}_2 \cdot \vec{v}_2 + 6 \hat{n} \times \vec{a}_1 \cdot \vec{S}_1 \hat{n} \cdot \vec{v}_2 \vec{v}_2 \cdot \vec{v}_2 \right) m_1 m_2 G^2 + \\
& \frac{1}{r^3} \left( 3 \hat{n} \times \vec{S}_1 \cdot \vec{v}_2 \vec{v}_1 \cdot \vec{v}_2 (\hat{n} \cdot \vec{v}_1)^2 - 3 \hat{n} \times \vec{S}_1 \cdot \vec{v}_1 \vec{v}_2 \cdot \vec{v}_2 (\hat{n} \cdot \vec{v}_1)^2 + 3 \vec{S}_1 \times \vec{v}_1 \cdot \vec{v}_2 \vec{v}_1 \cdot \vec{v}_2 \hat{n} \cdot \vec{v}_1 - \right. \\
& \left. 12 \hat{n} \times \vec{S}_1 \cdot \vec{v}_2 \hat{n} \cdot \vec{v}_2 \vec{v}_1 \cdot \vec{v}_2 \hat{n} \cdot \vec{v}_1 - 3 \vec{S}_1 \times \vec{v}_1 \cdot \vec{v}_2 \vec{v}_2 \cdot \vec{v}_2 \hat{n} \cdot \vec{v}_1 + 12 \hat{n} \times \vec{S}_1 \cdot \vec{v}_1 \hat{n} \cdot \vec{v}_2 \vec{v}_2 \cdot \vec{v}_2 \hat{n} \cdot \vec{v}_1 + \right.
\end{aligned}$$

$$3 \hat{n} \times \vec{S}_1 \cdot \vec{v}_2 (\vec{v}_1 \cdot \vec{v}_2)^2 - 6 \vec{S}_1 \times \vec{v}_1 \cdot \vec{v}_2 \hat{n} \cdot \vec{v}_2 \vec{v}_1 \cdot \vec{v}_2 - 3 \hat{n} \times \vec{S}_1 \cdot \vec{v}_1 \vec{v}_1 \cdot \vec{v}_2 \vec{v}_2 \cdot \vec{v}_2 \Big) m_1 m_2 G^2 \Big\}$$

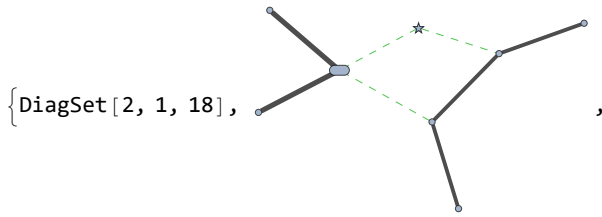

$$\begin{aligned} & \frac{1}{r^2} G^2 m_2^2 \left( 24 (\hat{n} \cdot \vec{v}_2)^2 \vec{S}_1 \times \vec{v}_2 \cdot \vec{a}_2 - 32 \hat{n} \cdot \vec{v}_1 \hat{n} \cdot \vec{v}_2 \vec{S}_1 \times \vec{v}_2 \cdot \vec{a}_2 - 8 \vec{a}_1 \cdot \vec{v}_2 \hat{n} \cdot \vec{v}_2 \hat{n} \times \vec{S}_1 \cdot \vec{v}_2 + \right. \\ & 8 \vec{v}_1 \cdot \vec{a}_2 \hat{n} \cdot \vec{v}_2 \hat{n} \times \vec{S}_1 \cdot \vec{v}_2 - 8 \vec{v}_1 \cdot \vec{v}_2 \hat{n} \cdot \vec{v}_2 \hat{n} \times \vec{S}_1 \cdot \vec{a}_2 - 8 \vec{v}_1 \cdot \vec{a}_2 \hat{n} \cdot \vec{v}_1 \hat{n} \times \vec{S}_1 \cdot \vec{v}_2 + 8 \vec{v}_1 \cdot \vec{v}_2 \hat{n} \cdot \vec{v}_1 \hat{n} \times \vec{S}_1 \cdot \vec{a}_2 - \\ & 4 \vec{v}_1 \cdot \vec{a}_2 \vec{S}_1 \times \vec{v}_1 \cdot \vec{v}_2 + 4 \vec{v}_1 \cdot \vec{v}_2 \vec{S}_1 \times \vec{v}_1 \cdot \vec{a}_2 + 16 \vec{v}_1 \cdot \vec{v}_2 \vec{S}_1 \times \vec{v}_2 \cdot \vec{a}_2 - 8 \vec{v}_1 \cdot \vec{v}_2 \hat{n} \cdot \vec{v}_2 \hat{n} \times \vec{S}_1 \cdot \vec{v}_2 \Big) + \frac{1}{r} \\ & G^2 m_2^2 \left( 16 \hat{n} \cdot \vec{v}_2 \vec{S}_1 \times \vec{v}_2 \cdot \vec{a}_2 + 4 \vec{a}_1 \cdot \vec{a}_2 \hat{n} \times \vec{S}_1 \cdot \vec{v}_2 - 4 \vec{a}_1 \cdot \vec{v}_2 \hat{n} \times \vec{S}_1 \cdot \vec{a}_2 + 4 \vec{v}_1 \cdot \vec{a}_2 \hat{n} \times \vec{S}_1 \cdot \vec{v}_2 - 4 \vec{v}_1 \cdot \vec{v}_2 \hat{n} \times \vec{S}_1 \cdot \vec{a}_2 \right) + \\ & G^2 m_2^2 \left( -4 \vec{S}_1 \times \vec{v}_2 \cdot \vec{a}_2 - 8 \vec{S}_1 \times \vec{a}_2 \cdot \vec{a}_2 \right) + \frac{1}{r^3} G^2 m_2^2 \\ & \left( -16 \vec{v}_1 \cdot \vec{v}_2 (\hat{n} \cdot \vec{v}_2)^2 \hat{n} \times \vec{S}_1 \cdot \vec{v}_2 + 8 \vec{v}_1 \cdot \vec{v}_2 \hat{n} \cdot \vec{v}_2 \vec{S}_1 \times \vec{v}_1 \cdot \vec{v}_2 + 32 \vec{v}_1 \cdot \vec{v}_2 \hat{n} \cdot \vec{v}_1 \hat{n} \cdot \vec{v}_2 \hat{n} \times \vec{S}_1 \cdot \vec{v}_2 - 8 (\vec{v}_1 \cdot \vec{v}_2)^2 \hat{n} \times \vec{S}_1 \cdot \vec{v}_2 \right) \Big\} \end{aligned}$$

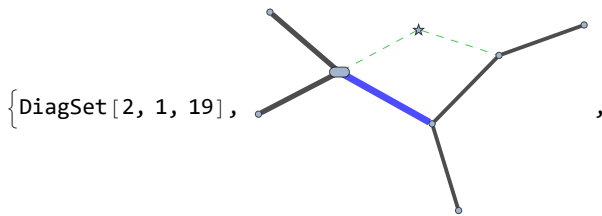

$$\begin{aligned} & \frac{1}{r^2} G^2 m_2^2 \left( 4 \hat{n} \cdot \vec{v}_1 \hat{n} \cdot \vec{v}_2 \vec{S}_1 \times \vec{v}_2 \cdot \vec{a}_2 - 4 \vec{v}_2 \cdot \vec{a}_2 \hat{n} \cdot \vec{v}_2 \hat{n} \times \vec{S}_1 \cdot \vec{v}_2 - 2 \vec{v}_2 \cdot \vec{v}_2 \hat{n} \cdot \vec{v}_2 \hat{n} \times \vec{S}_1 \cdot \vec{a}_2 - \right. \\ & 4 \vec{v}_2 \cdot \vec{a}_2 \hat{n} \cdot \vec{v}_1 \hat{n} \times \vec{S}_1 \cdot \vec{v}_2 + 8 \vec{v}_2 \cdot \vec{v}_2 \hat{n} \cdot \vec{v}_1 \hat{n} \times \vec{S}_1 \cdot \vec{a}_2 - 2 \vec{v}_1 \cdot \vec{v}_2 \vec{S}_1 \times \vec{v}_2 \cdot \vec{a}_2 - \\ & 2 \vec{v}_2 \cdot \vec{a}_2 \vec{S}_1 \times \vec{v}_1 \cdot \vec{v}_2 + 4 \vec{v}_2 \cdot \vec{v}_2 \vec{S}_1 \times \vec{v}_1 \cdot \vec{a}_2 - 2 \vec{v}_2 \cdot \vec{v}_2 \hat{n} \cdot \vec{v}_2 \hat{n} \times \vec{S}_1 \cdot \vec{v}_2 \Big) + \frac{1}{r} \\ & G^2 m_2^2 \left( -2 \hat{n} \cdot \vec{a}_2 \vec{S}_1 \times \vec{v}_2 \cdot \vec{a}_2 - 2 \hat{n} \cdot \vec{v}_2 \vec{S}_1 \times \vec{v}_2 \cdot \vec{a}_2 + 2 \vec{a}_2 \cdot \vec{a}_2 \hat{n} \times \vec{S}_1 \cdot \vec{v}_2 + 2 \vec{v}_2 \cdot \vec{a}_2 \hat{n} \times \vec{S}_1 \cdot \vec{v}_2 - \right. \\ & 6 \vec{v}_2 \cdot \vec{a}_2 \hat{n} \times \vec{S}_1 \cdot \vec{a}_2 - 4 \vec{v}_2 \cdot \vec{v}_2 \hat{n} \times \vec{S}_1 \cdot \vec{a}_2 \Big) + \frac{1}{r^3} G^2 m_2^2 \left( -2 \vec{v}_2 \cdot \vec{v}_2 (\hat{n} \cdot \vec{v}_2)^2 \hat{n} \times \vec{S}_1 \cdot \vec{v}_2 + \right. \\ & 2 \vec{v}_2 \cdot \vec{v}_2 \hat{n} \cdot \vec{v}_2 \vec{S}_1 \times \vec{v}_1 \cdot \vec{v}_2 + 8 \vec{v}_2 \cdot \vec{v}_2 \hat{n} \cdot \vec{v}_1 \hat{n} \cdot \vec{v}_2 \hat{n} \times \vec{S}_1 \cdot \vec{v}_2 - 2 \vec{v}_1 \cdot \vec{v}_2 \vec{v}_2 \cdot \vec{v}_2 \hat{n} \times \vec{S}_1 \cdot \vec{v}_2 \Big) \Big\} \end{aligned}$$

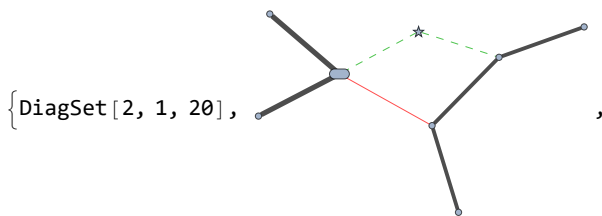

$$\begin{aligned} & \frac{1}{r^2} G^2 m_2^2 \left( 4 (\hat{n} \cdot \vec{v}_2)^2 \vec{S}_1 \times \vec{a}_1 \cdot \vec{v}_2 - 12 (\hat{n} \cdot \vec{v}_2)^2 \vec{S}_1 \times \vec{v}_1 \cdot \vec{a}_2 + 4 \hat{n} \cdot \vec{a}_2 \hat{n} \cdot \vec{v}_2 \vec{S}_1 \times \vec{v}_1 \cdot \vec{v}_2 + 8 \hat{n} \cdot \vec{v}_1 \hat{n} \cdot \vec{v}_2 \vec{S}_1 \times \vec{v}_1 \cdot \vec{a}_2 + \right. \\ & 16 \vec{v}_2 \cdot \vec{a}_2 \hat{n} \cdot \vec{v}_2 \hat{n} \times \vec{S}_1 \cdot \vec{v}_2 + 8 \vec{v}_2 \cdot \vec{v}_2 \hat{n} \cdot \vec{v}_2 \hat{n} \times \vec{S}_1 \cdot \vec{a}_2 - 8 \vec{v}_2 \cdot \vec{a}_2 \hat{n} \cdot \vec{v}_1 \hat{n} \times \vec{S}_1 \cdot \vec{v}_2 - 16 \vec{v}_2 \cdot \vec{v}_2 \hat{n} \cdot \vec{v}_1 \hat{n} \times \vec{S}_1 \cdot \vec{a}_2 - \\ & 4 \vec{v}_1 \cdot \vec{v}_2 \vec{S}_1 \times \vec{v}_1 \cdot \vec{a}_2 - 4 \vec{v}_2 \cdot \vec{a}_2 \vec{S}_1 \times \vec{v}_1 \cdot \vec{v}_2 - 4 \vec{v}_2 \cdot \vec{v}_2 \vec{S}_1 \times \vec{v}_1 \cdot \vec{a}_2 + 4 (\hat{n} \cdot \vec{v}_2)^2 \vec{S}_1 \times \vec{v}_1 \cdot \vec{v}_2 + 8 \vec{v}_2 \cdot \vec{v}_2 \hat{n} \cdot \vec{v}_2 \hat{n} \times \vec{S}_1 \cdot \vec{v}_2 \Big) + \\ & \frac{1}{r} G^2 m_2^2 \left( -4 \hat{n} \cdot \vec{a}_2 \vec{S}_1 \times \vec{v}_1 \cdot \vec{a}_2 - 4 \hat{n} \cdot \vec{v}_2 \vec{S}_1 \times \vec{v}_1 \cdot \vec{a}_2 - 4 \hat{n} \cdot \vec{v}_2 \vec{S}_1 \times \vec{a}_1 \cdot \vec{a}_2 + 4 \vec{v}_2 \cdot \vec{a}_2 \hat{n} \times \vec{S}_1 \cdot \vec{v}_2 + \right. \end{aligned}$$

$$12 \vec{v}_2 \cdot \vec{a}_2 \hat{n} \times \vec{S}_1 \cdot \vec{a}_2 + 8 \vec{v}_2 \cdot \vec{v}_2 \hat{n} \times \vec{S}_1 \cdot \vec{a}_2 \Big) + \frac{1}{r^3} \\ G^2 m_2^2 \left( 12 (\hat{n} \cdot \vec{v}_2)^3 \vec{S}_1 \times \vec{v}_1 \cdot \vec{v}_2 - 16 \hat{n} \cdot \vec{v}_1 (\hat{n} \cdot \vec{v}_2)^2 \vec{S}_1 \times \vec{v}_1 \cdot \vec{v}_2 + 8 \vec{v}_2 \cdot \vec{v}_2 (\hat{n} \cdot \vec{v}_2)^2 \hat{n} \times \vec{S}_1 \cdot \vec{v}_2 + 8 \vec{v}_1 \cdot \vec{v}_2 \hat{n} \cdot \vec{v}_2 \vec{S}_1 \times \vec{v}_1 \cdot \vec{v}_2 - \right. \\ \left. 12 \vec{v}_2 \cdot \vec{v}_2 \hat{n} \cdot \vec{v}_2 \vec{S}_1 \times \vec{v}_1 \cdot \vec{v}_2 - 32 \vec{v}_2 \cdot \vec{v}_2 \hat{n} \cdot \vec{v}_1 \hat{n} \cdot \vec{v}_2 \hat{n} \times \vec{S}_1 \cdot \vec{v}_2 + 8 \vec{v}_1 \cdot \vec{v}_2 \vec{v}_2 \cdot \vec{v}_2 \hat{n} \times \vec{S}_1 \cdot \vec{v}_2 \right) \Big\}$$

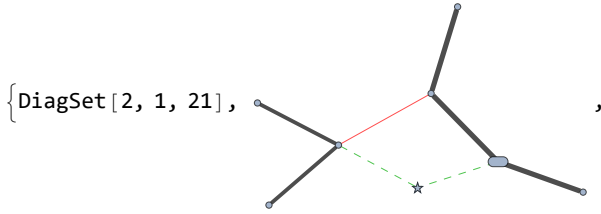

$$\left( 2 \vec{a}_1 \times \vec{a}_2 \cdot \vec{S}_1 + 4 \vec{a}_1 \times \vec{a}_2 \cdot \vec{S}_1 + 2 \vec{a}_2 \times \vec{S}_1 \cdot \vec{v}_1 \right) m_1 m_2 G^2 + \frac{1}{r} \left( \frac{1}{2} \vec{a}_2 \times \vec{S}_1 \cdot \vec{v}_1 \hat{n} \cdot \vec{a}_1 + 2 \vec{a}_1 \times \vec{S}_1 \cdot \vec{v}_2 \hat{n} \cdot \vec{v}_1 - 2 \vec{S}_1 \times \vec{v}_1 \cdot \vec{v}_2 \hat{n} \cdot \vec{v}_1 + \right. \\ \left. 4 \vec{a}_1 \times \vec{S}_1 \cdot \vec{v}_2 \hat{n} \cdot \vec{v}_1 + \frac{5}{2} \vec{a}_1 \times \vec{a}_2 \cdot \vec{S}_1 \hat{n} \cdot \vec{v}_1 + \frac{5}{2} \vec{a}_2 \times \vec{S}_1 \cdot \vec{v}_1 \hat{n} \cdot \vec{v}_1 + \frac{3}{2} \hat{n} \times \vec{S}_1 \cdot \vec{v}_1 \vec{a}_1 \cdot \vec{a}_2 + 3 \hat{n} \times \vec{S}_1 \cdot \vec{v}_2 \vec{a}_1 \cdot \vec{v}_1 + \right. \\ \left. \frac{3}{2} \hat{n} \times \vec{S}_1 \cdot \vec{v}_1 \vec{a}_2 \cdot \vec{v}_1 - \frac{3}{2} \hat{n} \times \vec{a}_1 \cdot \vec{S}_1 \vec{a}_2 \cdot \vec{v}_1 - 3 \hat{n} \times \vec{S}_1 \cdot \vec{v}_2 \vec{a}_2 \cdot \vec{v}_2 - \frac{3}{2} \hat{n} \times \vec{a}_2 \cdot \vec{S}_1 \vec{v}_1 \cdot \vec{v}_1 + \frac{3}{2} \hat{n} \times \vec{a}_2 \cdot \vec{S}_1 \vec{v}_2 \cdot \vec{v}_2 \right) m_1 m_2 G^2 + \\ \frac{1}{r^2} \left( -\frac{5}{2} \vec{S}_1 \times \vec{v}_1 \cdot \vec{v}_2 (\hat{n} \cdot \vec{v}_1)^2 + \frac{5}{2} \vec{a}_1 \times \vec{S}_1 \cdot \vec{v}_2 (\hat{n} \cdot \vec{v}_1)^2 - \frac{1}{2} \vec{a}_2 \times \vec{S}_1 \cdot \vec{v}_1 (\hat{n} \cdot \vec{v}_1)^2 - \frac{1}{2} \vec{S}_1 \times \vec{v}_1 \cdot \vec{v}_2 \hat{n} \cdot \vec{a}_1 \hat{n} \cdot \vec{v}_1 + \right. \\ \left. 5 \vec{S}_1 \times \vec{v}_1 \cdot \vec{v}_2 \hat{n} \cdot \vec{v}_2 \hat{n} \cdot \vec{v}_1 - 5 \vec{a}_1 \times \vec{S}_1 \cdot \vec{v}_2 \hat{n} \cdot \vec{v}_2 \hat{n} \cdot \vec{v}_1 - 3 \hat{n} \times \vec{S}_1 \cdot \vec{v}_2 \vec{a}_1 \cdot \vec{v}_1 \hat{n} \cdot \vec{v}_1 - \frac{3}{2} \hat{n} \times \vec{S}_1 \cdot \vec{v}_1 \vec{a}_1 \cdot \vec{v}_2 \hat{n} \cdot \vec{v}_1 - \right. \\ \left. \frac{3}{2} \hat{n} \times \vec{S}_1 \cdot \vec{v}_1 \vec{a}_2 \cdot \vec{v}_1 \hat{n} \cdot \vec{v}_1 + 3 \hat{n} \times \vec{S}_1 \cdot \vec{v}_2 \vec{a}_2 \cdot \vec{v}_2 \hat{n} \cdot \vec{v}_1 - \frac{3}{2} \hat{n} \times \vec{S}_1 \cdot \vec{v}_2 \vec{v}_1 \cdot \vec{v}_1 \hat{n} \cdot \vec{v}_1 + \frac{3}{2} \hat{n} \times \vec{a}_2 \cdot \vec{S}_1 \vec{v}_1 \cdot \vec{v}_1 \hat{n} \cdot \vec{v}_1 - \right. \\ \left. \frac{3}{2} \hat{n} \times \vec{S}_1 \cdot \vec{v}_1 \vec{v}_1 \cdot \vec{v}_2 \hat{n} \cdot \vec{v}_1 + \frac{3}{2} \hat{n} \times \vec{a}_1 \cdot \vec{S}_1 \vec{v}_1 \cdot \vec{v}_2 \hat{n} \cdot \vec{v}_1 + \frac{3}{2} \hat{n} \times \vec{S}_1 \cdot \vec{v}_2 \vec{v}_2 \cdot \vec{v}_2 \hat{n} \cdot \vec{v}_1 - \frac{3}{2} \hat{n} \times \vec{a}_2 \cdot \vec{S}_1 \vec{v}_2 \cdot \vec{v}_2 \hat{n} \cdot \vec{v}_1 + \right. \\ \left. \vec{S}_1 \times \vec{v}_1 \cdot \vec{v}_2 \hat{n} \cdot \vec{a}_1 \hat{n} \cdot \vec{v}_2 - 3 \vec{S}_1 \times \vec{v}_1 \cdot \vec{v}_2 \vec{a}_1 \cdot \vec{v}_1 - 2 \vec{S}_1 \times \vec{v}_1 \cdot \vec{v}_2 \vec{a}_1 \cdot \vec{v}_2 + 3 \hat{n} \times \vec{S}_1 \cdot \vec{v}_1 \hat{n} \cdot \vec{v}_2 \vec{a}_1 \cdot \vec{v}_2 + \right. \\ \left. 3 \vec{S}_1 \times \vec{v}_1 \cdot \vec{v}_2 \vec{a}_2 \cdot \vec{v}_2 - \vec{a}_2 \times \vec{S}_1 \cdot \vec{v}_1 \vec{v}_1 \cdot \vec{v}_1 + 3 \hat{n} \times \vec{S}_1 \cdot \vec{v}_2 \hat{n} \cdot \vec{v}_2 \vec{v}_1 \cdot \vec{v}_1 - 4 \vec{S}_1 \times \vec{v}_1 \cdot \vec{v}_2 \vec{v}_1 \cdot \vec{v}_2 + 4 \vec{a}_1 \times \vec{S}_1 \cdot \vec{v}_2 \vec{v}_1 \cdot \vec{v}_2 + \right. \\ \left. 3 \hat{n} \times \vec{S}_1 \cdot \vec{v}_1 \hat{n} \cdot \vec{v}_2 \vec{v}_1 \cdot \vec{v}_2 - 3 \hat{n} \times \vec{a}_1 \cdot \vec{S}_1 \hat{n} \cdot \vec{v}_2 \vec{v}_1 \cdot \vec{v}_2 + \frac{3}{2} \vec{a}_2 \times \vec{S}_1 \cdot \vec{v}_1 \vec{v}_2 \cdot \vec{v}_2 - 3 \hat{n} \times \vec{S}_1 \cdot \vec{v}_2 \hat{n} \cdot \vec{v}_2 \vec{v}_2 \cdot \vec{v}_2 \right) m_1 m_2 G^2 + \\ \frac{1}{r^3} \left( \frac{1}{2} \vec{S}_1 \times \vec{v}_1 \cdot \vec{v}_2 (\hat{n} \cdot \vec{v}_1)^3 - 2 \vec{S}_1 \times \vec{v}_1 \cdot \vec{v}_2 \hat{n} \cdot \vec{v}_2 (\hat{n} \cdot \vec{v}_1)^2 + \frac{3}{2} \hat{n} \times \vec{S}_1 \cdot \vec{v}_2 \vec{v}_1 \cdot \vec{v}_1 (\hat{n} \cdot \vec{v}_1)^2 + \right. \\ \left. \frac{3}{2} \hat{n} \times \vec{S}_1 \cdot \vec{v}_1 \vec{v}_1 \cdot \vec{v}_2 (\hat{n} \cdot \vec{v}_1)^2 - \frac{3}{2} \hat{n} \times \vec{S}_1 \cdot \vec{v}_2 \vec{v}_2 \cdot \vec{v}_2 (\hat{n} \cdot \vec{v}_1)^2 + \vec{S}_1 \times \vec{v}_1 \cdot \vec{v}_2 \vec{v}_1 \cdot \vec{v}_1 \hat{n} \cdot \vec{v}_1 - \right. \\ \left. 6 \hat{n} \times \vec{S}_1 \cdot \vec{v}_2 \hat{n} \cdot \vec{v}_2 \vec{v}_1 \cdot \vec{v}_1 \hat{n} \cdot \vec{v}_1 + \frac{5}{2} \vec{S}_1 \times \vec{v}_1 \cdot \vec{v}_2 \vec{v}_1 \cdot \vec{v}_2 \hat{n} \cdot \vec{v}_1 - 6 \hat{n} \times \vec{S}_1 \cdot \vec{v}_1 \hat{n} \cdot \vec{v}_2 \vec{v}_1 \cdot \vec{v}_2 \hat{n} \cdot \vec{v}_1 - \right. \\ \left. \frac{3}{2} \vec{S}_1 \times \vec{v}_1 \cdot \vec{v}_2 \vec{v}_2 \cdot \vec{v}_2 \hat{n} \cdot \vec{v}_1 + 6 \hat{n} \times \vec{S}_1 \cdot \vec{v}_2 \hat{n} \cdot \vec{v}_2 \vec{v}_2 \cdot \vec{v}_2 \hat{n} \cdot \vec{v}_1 + \frac{3}{2} \hat{n} \times \vec{S}_1 \cdot \vec{v}_1 (\vec{v}_1 \cdot \vec{v}_2)^2 - 2 \vec{S}_1 \times \vec{v}_1 \cdot \vec{v}_2 \hat{n} \cdot \vec{v}_2 \vec{v}_1 \cdot \vec{v}_1 + \right. \\ \left. \frac{3}{2} \hat{n} \times \vec{S}_1 \cdot \vec{v}_2 \vec{v}_1 \cdot \vec{v}_1 \vec{v}_1 \cdot \vec{v}_2 + 3 \vec{S}_1 \times \vec{v}_1 \cdot \vec{v}_2 \hat{n} \cdot \vec{v}_2 \vec{v}_2 \cdot \vec{v}_2 - \frac{3}{2} \hat{n} \times \vec{S}_1 \cdot \vec{v}_2 \vec{v}_1 \cdot \vec{v}_2 \vec{v}_2 \cdot \vec{v}_2 \right) m_1 m_2 G^2 \Big\}$$

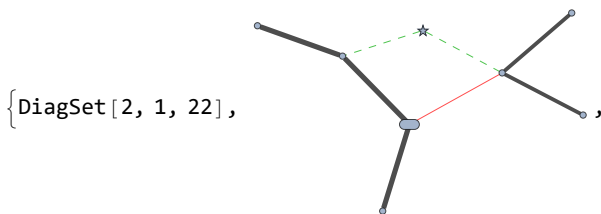

$$\frac{1}{r^2} G^2 m_1 m_2 \left( 12 \vec{a}_1 \cdot \vec{v}_2 \hat{n} \cdot \vec{v}_1 \hat{n} \times \vec{S}_1 \cdot \vec{v}_1 - 8 \vec{a}_1 \cdot \vec{v}_2 \hat{n} \cdot \vec{v}_2 \hat{n} \times \vec{S}_1 \cdot \vec{v}_1 - \right. \\ \left. 4 \vec{a}_2 \cdot \vec{v}_1 \hat{n} \cdot \vec{v}_1 \hat{n} \times \vec{S}_1 \cdot \vec{v}_1 + 4 \vec{v}_1 \cdot \vec{v}_2 \hat{n} \cdot \vec{v}_1 \hat{n} \times \vec{a}_1 \cdot \vec{S}_1 + 4 \vec{a}_1 \cdot \vec{v}_2 \vec{S}_1 \times \vec{v}_1 \cdot \vec{v}_2 - 4 \vec{v}_1 \cdot \vec{v}_2 \hat{n} \cdot \vec{v}_1 \hat{n} \times \vec{S}_1 \cdot \vec{v}_1 \right) +$$



$$\frac{G^2 m_1 m_2 \left( -4 \vec{a}_1 \cdot \vec{a}_2 \hat{n} \times \vec{S}_1 \cdot \vec{v}_1 - 4 \vec{a}_1 \cdot \vec{v}_2 \hat{n} \times \vec{S}_1 \cdot \vec{v}_1 + 4 \vec{a}_1 \cdot \vec{v}_2 \hat{n} \times \vec{a}_1 \cdot \vec{S}_1 \right)}{r} + \frac{1}{r^3} G^2 m_1 m_2 \left( 12 \vec{v}_1 \cdot \vec{v}_2 (\hat{n} \cdot \vec{v}_1)^2 \hat{n} \times \vec{S}_1 \cdot \vec{v}_1 + 4 \vec{v}_1 \cdot \vec{v}_2 \hat{n} \cdot \vec{v}_1 \vec{S}_1 \times \vec{v}_1 \cdot \vec{v}_2 - 16 \vec{v}_1 \cdot \vec{v}_2 \hat{n} \cdot \vec{v}_2 \hat{n} \cdot \vec{v}_1 \hat{n} \times \vec{S}_1 \cdot \vec{v}_1 + 4 (\vec{v}_1 \cdot \vec{v}_2)^2 \hat{n} \times \vec{S}_1 \cdot \vec{v}_1 \right) \}$$

{DiagSet[2, 1, 23], 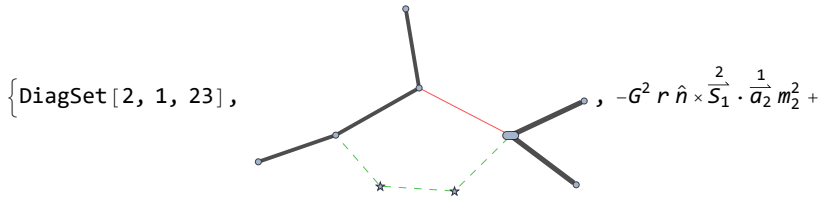 ,  $-G^2 r \hat{n} \times \vec{S}_1 \cdot \frac{2}{\vec{a}_2} \cdot \frac{1}{\vec{a}_2} m_2^2 +$

$$\begin{aligned} & G^2 \left( 2 \vec{S}_1 \times \vec{v}_1 \cdot \frac{1}{\vec{a}_2} - \vec{S}_1 \times \vec{v}_2 \cdot \vec{a}_2 + \vec{S}_1 \times \vec{a}_1 \cdot \frac{1}{\vec{a}_2} + \hat{n} \times \vec{S}_1 \cdot \vec{v}_2 \hat{n} \cdot \vec{a}_2 - \hat{n} \times \vec{S}_1 \cdot \frac{1}{\vec{a}_2} \hat{n} \cdot \vec{a}_2 - 2 \hat{n} \times \vec{S}_1 \cdot \frac{1}{\vec{a}_2} \hat{n} \cdot \vec{v}_2 + 2 \hat{n} \times \vec{S}_1 \cdot \vec{a}_2 \hat{n} \cdot \vec{v}_2 \right) \\ & m_2^2 + \frac{1}{r} G^2 \left( \hat{n} \times \vec{S}_1 \cdot \vec{v}_2 (\hat{n} \cdot \vec{a}_2)^2 - 2 \vec{S}_1 \times \vec{v}_1 \cdot \vec{v}_2 \hat{n} \cdot \vec{a}_2 - \vec{S}_1 \times \vec{a}_1 \cdot \vec{v}_2 \hat{n} \cdot \vec{a}_2 - \vec{S}_1 \times \vec{v}_2 \cdot \vec{a}_2 \hat{n} \cdot \vec{a}_2 - \right. \\ & 2 \hat{n} \times \vec{S}_1 \cdot \vec{v}_2 \hat{n} \cdot \vec{a}_1 \hat{n} \cdot \vec{a}_2 - 4 \hat{n} \times \vec{S}_1 \cdot \vec{v}_2 \hat{n} \cdot \vec{v}_1 \hat{n} \cdot \vec{a}_2 + 2 \hat{n} \times \vec{S}_1 \cdot \vec{v}_2 \hat{n} \cdot \vec{v}_2 \hat{n} \cdot \vec{a}_2 + 2 \hat{n} \times \vec{S}_1 \cdot \vec{a}_2 \hat{n} \cdot \vec{v}_2 \hat{n} \cdot \vec{a}_2 + \\ & 4 \hat{n} \times \vec{S}_1 \cdot \vec{a}_2 (\hat{n} \cdot \vec{v}_2)^2 + \hat{n} \times \vec{S}_1 \cdot \vec{v}_2 (\hat{n} \cdot \vec{v}_2)^2 - 3 \hat{n} \times \vec{S}_1 \cdot \frac{1}{\vec{a}_2} (\hat{n} \cdot \vec{v}_2)^2 - 4 \vec{S}_1 \times \vec{v}_1 \cdot \vec{a}_2 \hat{n} \cdot \vec{v}_2 - \\ & 2 \vec{S}_1 \times \vec{v}_2 \cdot \vec{a}_2 \hat{n} \cdot \vec{v}_2 - 2 \vec{S}_1 \times \vec{a}_1 \cdot \vec{a}_2 \hat{n} \cdot \vec{v}_2 + 2 \vec{S}_1 \times \vec{v}_1 \cdot \frac{1}{\vec{a}_2} \hat{n} \cdot \vec{v}_2 - 4 \hat{n} \times \vec{S}_1 \cdot \vec{a}_2 \hat{n} \cdot \vec{a}_1 \hat{n} \cdot \vec{v}_2 - \\ & 8 \hat{n} \times \vec{S}_1 \cdot \vec{a}_2 \hat{n} \cdot \vec{v}_1 \hat{n} \cdot \vec{v}_2 + 4 \hat{n} \times \vec{S}_1 \cdot \frac{1}{\vec{a}_2} \hat{n} \cdot \vec{v}_1 \hat{n} \cdot \vec{v}_2 + \hat{n} \times \vec{S}_1 \cdot \vec{v}_2 \vec{a}_1 \cdot \vec{a}_2 + 2 \hat{n} \times \vec{S}_1 \cdot \vec{a}_2 \vec{a}_1 \cdot \vec{v}_2 + \\ & 2 \hat{n} \times \vec{S}_1 \cdot \vec{v}_2 \vec{v}_1 \cdot \vec{a}_2 + 4 \hat{n} \times \vec{S}_1 \cdot \vec{a}_2 \vec{v}_1 \cdot \vec{v}_2 - 2 \hat{n} \times \vec{S}_1 \cdot \frac{1}{\vec{a}_2} \vec{v}_1 \cdot \vec{v}_2 - \hat{n} \times \vec{S}_1 \cdot \vec{v}_2 \vec{v}_2 \cdot \vec{v}_2 + \hat{n} \times \vec{S}_1 \cdot \frac{1}{\vec{a}_2} \vec{v}_2 \cdot \vec{v}_2 \left. \right) m_2^2 + \\ & \frac{1}{r^2} G^2 \left( 2 \hat{n} \times \vec{S}_1 \cdot \vec{v}_2 (\hat{n} \cdot \vec{v}_2)^3 + 6 \hat{n} \times \vec{S}_1 \cdot \vec{a}_2 (\hat{n} \cdot \vec{v}_2)^3 - 2 \vec{S}_1 \times \vec{v}_1 \cdot \vec{v}_2 (\hat{n} \cdot \vec{v}_2)^2 - \vec{S}_1 \times \vec{a}_1 \cdot \vec{v}_2 (\hat{n} \cdot \vec{v}_2)^2 - \right. \\ & 4 \vec{S}_1 \times \vec{v}_1 \cdot \vec{a}_2 (\hat{n} \cdot \vec{v}_2)^2 - 3 \vec{S}_1 \times \vec{v}_2 \cdot \vec{a}_2 (\hat{n} \cdot \vec{v}_2)^2 - 4 \hat{n} \times \vec{S}_1 \cdot \vec{v}_2 \hat{n} \cdot \vec{a}_1 (\hat{n} \cdot \vec{v}_2)^2 + 4 \hat{n} \times \vec{S}_1 \cdot \vec{v}_2 \hat{n} \cdot \vec{a}_2 (\hat{n} \cdot \vec{v}_2)^2 - \\ & 8 \hat{n} \times \vec{S}_1 \cdot \frac{1}{\vec{a}_2} \hat{n} \cdot \vec{v}_1 (\hat{n} \cdot \vec{v}_2)^2 - 16 \hat{n} \times \vec{S}_1 \cdot \vec{a}_2 \hat{n} \cdot \vec{v}_1 (\hat{n} \cdot \vec{v}_2)^2 + 16 \hat{n} \times \vec{S}_1 \cdot \vec{a}_2 (\hat{n} \cdot \vec{v}_1)^2 \hat{n} \cdot \vec{v}_2 - 2 \vec{S}_1 \times \vec{v}_1 \cdot \vec{v}_2 \hat{n} \cdot \vec{a}_2 \hat{n} \cdot \vec{v}_2 + \\ & 8 \vec{S}_1 \times \vec{v}_1 \cdot \vec{a}_2 \hat{n} \cdot \vec{v}_1 \hat{n} \cdot \vec{v}_2 + 4 \vec{S}_1 \times \vec{v}_2 \cdot \vec{a}_2 \hat{n} \cdot \vec{v}_1 \hat{n} \cdot \vec{v}_2 - 8 \hat{n} \times \vec{S}_1 \cdot \vec{v}_2 \hat{n} \cdot \vec{a}_2 \hat{n} \cdot \vec{v}_1 \hat{n} \cdot \vec{v}_2 + 2 \hat{n} \times \vec{S}_1 \cdot \vec{v}_2 \vec{a}_1 \cdot \vec{v}_2 \hat{n} \cdot \vec{v}_2 + \\ & 2 \hat{n} \times \vec{S}_1 \cdot \vec{v}_2 \vec{v}_1 \cdot \vec{a}_2 \hat{n} \cdot \vec{v}_2 - 4 \hat{n} \times \vec{S}_1 \cdot \vec{a}_2 \vec{v}_1 \cdot \vec{v}_1 \hat{n} \cdot \vec{v}_2 + 4 \hat{n} \times \vec{S}_1 \cdot \frac{1}{\vec{a}_2} \vec{v}_1 \cdot \vec{v}_2 \hat{n} \cdot \vec{v}_2 + 8 \hat{n} \times \vec{S}_1 \cdot \vec{a}_2 \vec{v}_1 \cdot \vec{v}_2 \hat{n} \cdot \vec{v}_2 - \\ & 2 \hat{n} \times \vec{S}_1 \cdot \vec{v}_2 \vec{v}_2 \cdot \vec{v}_2 \hat{n} \cdot \vec{v}_2 - 2 \hat{n} \times \vec{S}_1 \cdot \vec{a}_2 \vec{v}_2 \cdot \vec{v}_2 \hat{n} \cdot \vec{v}_2 + 8 \hat{n} \times \vec{S}_1 \cdot \vec{v}_2 \hat{n} \cdot \vec{a}_2 (\hat{n} \cdot \vec{v}_1)^2 + 4 \vec{S}_1 \times \vec{v}_1 \cdot \vec{v}_2 \hat{n} \cdot \vec{a}_2 \hat{n} \cdot \vec{v}_1 - \\ & 2 \vec{S}_1 \times \vec{v}_1 \cdot \vec{v}_2 \vec{v}_1 \cdot \vec{a}_2 - 4 \hat{n} \times \vec{S}_1 \cdot \vec{v}_2 \hat{n} \cdot \vec{v}_1 \vec{v}_1 \cdot \vec{a}_2 - 2 \hat{n} \times \vec{S}_1 \cdot \vec{v}_2 \hat{n} \cdot \vec{a}_2 \vec{v}_1 \cdot \vec{v}_1 - 4 \vec{S}_1 \times \vec{v}_1 \cdot \vec{a}_2 \vec{v}_1 \cdot \vec{v}_2 - \\ & 2 \vec{S}_1 \times \vec{v}_2 \cdot \vec{a}_2 \vec{v}_1 \cdot \vec{v}_2 + 2 \hat{n} \times \vec{S}_1 \cdot \vec{v}_2 \hat{n} \cdot \vec{a}_2 \vec{v}_1 \cdot \vec{v}_2 - 8 \hat{n} \times \vec{S}_1 \cdot \vec{a}_2 \hat{n} \cdot \vec{v}_1 \vec{v}_1 \cdot \vec{v}_2 + 2 \vec{S}_1 \times \vec{v}_1 \cdot \vec{v}_2 \vec{v}_2 \cdot \vec{v}_2 + \vec{S}_1 \times \vec{a}_1 \cdot \vec{v}_2 \vec{v}_2 \cdot \vec{v}_2 + \\ & \vec{S}_1 \times \vec{v}_2 \cdot \vec{a}_2 \vec{v}_2 \cdot \vec{v}_2 + 2 \hat{n} \times \vec{S}_1 \cdot \vec{v}_2 \hat{n} \cdot \vec{a}_1 \vec{v}_2 \cdot \vec{v}_2 - 2 \hat{n} \times \vec{S}_1 \cdot \vec{v}_2 \hat{n} \cdot \vec{a}_2 \vec{v}_2 \cdot \vec{v}_2 + 4 \hat{n} \times \vec{S}_1 \cdot \frac{1}{\vec{a}_2} \vec{v}_2 \hat{n} \cdot \vec{v}_1 \vec{v}_2 \cdot \vec{v}_2 \left. \right) m_2^2 + \frac{1}{r^3} \\ & G^2 \left( 3 \hat{n} \times \vec{S}_1 \cdot \vec{v}_2 (\hat{n} \cdot \vec{v}_2)^4 - 2 \vec{S}_1 \times \vec{v}_1 \cdot \vec{v}_2 (\hat{n} \cdot \vec{v}_2)^3 - 12 \hat{n} \times \vec{S}_1 \cdot \vec{v}_2 \hat{n} \cdot \vec{v}_1 (\hat{n} \cdot \vec{v}_2)^3 + 24 \hat{n} \times \vec{S}_1 \cdot \vec{v}_2 (\hat{n} \cdot \vec{v}_1)^2 (\hat{n} \cdot \vec{v}_2)^2 + \right. \\ & 8 \vec{S}_1 \times \vec{v}_1 \cdot \vec{v}_2 \hat{n} \cdot \vec{v}_1 (\hat{n} \cdot \vec{v}_2)^2 - 4 \hat{n} \times \vec{S}_1 \cdot \vec{v}_2 \vec{v}_1 \cdot \vec{v}_1 (\hat{n} \cdot \vec{v}_2)^2 + 6 \hat{n} \times \vec{S}_1 \cdot \vec{v}_2 \vec{v}_1 \cdot \vec{v}_2 (\hat{n} \cdot \vec{v}_2)^2 - \\ & 4 \hat{n} \times \vec{S}_1 \cdot \vec{v}_2 \vec{v}_2 \cdot \vec{v}_2 (\hat{n} \cdot \vec{v}_2)^2 - 4 \vec{S}_1 \times \vec{v}_1 \cdot \vec{v}_2 \vec{v}_1 \cdot \vec{v}_2 \hat{n} \cdot \vec{v}_2 - 16 \hat{n} \times \vec{S}_1 \cdot \vec{v}_2 \hat{n} \cdot \vec{v}_1 \vec{v}_1 \cdot \vec{v}_2 \hat{n} \cdot \vec{v}_2 + \\ & 2 \vec{S}_1 \times \vec{v}_1 \cdot \vec{v}_2 \vec{v}_2 \cdot \vec{v}_2 \hat{n} \cdot \vec{v}_2 + 8 \hat{n} \times \vec{S}_1 \cdot \vec{v}_2 \hat{n} \cdot \vec{v}_1 \vec{v}_2 \cdot \vec{v}_2 \hat{n} \cdot \vec{v}_2 + 2 \hat{n} \times \vec{S}_1 \cdot \vec{v}_2 (\vec{v}_1 \cdot \vec{v}_2)^2 + \hat{n} \times \vec{S}_1 \cdot \vec{v}_2 (\vec{v}_2 \cdot \vec{v}_2)^2 - \\ & 8 \hat{n} \times \vec{S}_1 \cdot \vec{v}_2 (\hat{n} \cdot \vec{v}_1)^2 \vec{v}_2 \cdot \vec{v}_2 - 4 \vec{S}_1 \times \vec{v}_1 \cdot \vec{v}_2 \hat{n} \cdot \vec{v}_1 \vec{v}_2 \cdot \vec{v}_2 + 2 \hat{n} \times \vec{S}_1 \cdot \vec{v}_2 \vec{v}_1 \cdot \vec{v}_1 \vec{v}_2 \cdot \vec{v}_2 - 2 \hat{n} \times \vec{S}_1 \cdot \vec{v}_2 \vec{v}_1 \cdot \vec{v}_2 \vec{v}_2 \cdot \vec{v}_2 \left. \right) m_2^2 \} \end{aligned}$$

{DiagSet[2, 1, 24], 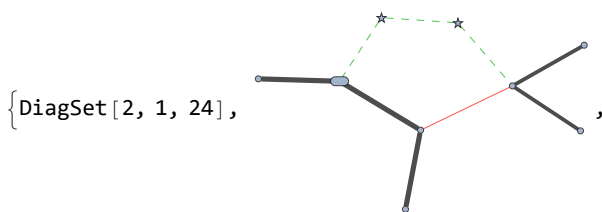 ,

$$\begin{aligned} & \left( \frac{3}{4} \hat{n} \times \vec{S}_1 \cdot \vec{v}_2 \left( \hat{n} \cdot \vec{v}_1 \right)^4 + \frac{3}{2} \vec{S}_1 \times \vec{v}_1 \cdot \vec{v}_2 \left( \hat{n} \cdot \vec{v}_1 \right)^3 - 3 \hat{n} \times \vec{S}_1 \cdot \vec{v}_2 \hat{n} \cdot \vec{v}_2 \left( \hat{n} \cdot \vec{v}_1 \right)^3 + 6 \hat{n} \times \vec{S}_1 \cdot \vec{v}_2 \left( \hat{n} \cdot \vec{v}_2 \right)^2 \left( \hat{n} \cdot \vec{v}_1 \right)^2 - \right. \\ & 4 \vec{S}_1 \times \vec{v}_1 \cdot \vec{v}_2 \hat{n} \cdot \vec{v}_2 \left( \hat{n} \cdot \vec{v}_1 \right)^2 - \hat{n} \times \vec{S}_1 \cdot \vec{v}_2 \vec{v}_1 \cdot \vec{v}_1 \left( \hat{n} \cdot \vec{v}_1 \right)^2 + \frac{3}{2} \hat{n} \times \vec{S}_1 \cdot \vec{v}_2 \vec{v}_1 \cdot \vec{v}_2 \left( \hat{n} \cdot \vec{v}_1 \right)^2 - \\ & \hat{n} \times \vec{S}_1 \cdot \vec{v}_2 \vec{v}_2 \cdot \vec{v}_2 \left( \hat{n} \cdot \vec{v}_1 \right)^2 + 4 \vec{S}_1 \times \vec{v}_1 \cdot \vec{v}_2 \left( \hat{n} \cdot \vec{v}_2 \right)^2 \hat{n} \cdot \vec{v}_1 - \frac{1}{2} \vec{S}_1 \times \vec{v}_1 \cdot \vec{v}_2 \vec{v}_1 \cdot \vec{v}_1 \hat{n} \cdot \vec{v}_1 + \\ & 2 \hat{n} \times \vec{S}_1 \cdot \vec{v}_2 \hat{n} \cdot \vec{v}_2 \vec{v}_1 \cdot \vec{v}_1 \hat{n} \cdot \vec{v}_1 + 2 \vec{S}_1 \times \vec{v}_1 \cdot \vec{v}_2 \vec{v}_1 \cdot \vec{v}_2 \hat{n} \cdot \vec{v}_1 - 4 \hat{n} \times \vec{S}_1 \cdot \vec{v}_2 \hat{n} \cdot \vec{v}_2 \vec{v}_1 \cdot \vec{v}_2 \hat{n} \cdot \vec{v}_1 - \\ & \vec{S}_1 \times \vec{v}_1 \cdot \vec{v}_2 \vec{v}_2 \cdot \vec{v}_2 \hat{n} \cdot \vec{v}_1 + \frac{1}{4} \hat{n} \times \vec{S}_1 \cdot \vec{v}_2 \left( \vec{v}_1 \cdot \vec{v}_1 \right)^2 + \frac{1}{2} \hat{n} \times \vec{S}_1 \cdot \vec{v}_2 \left( \vec{v}_1 \cdot \vec{v}_2 \right)^2 - 2 \hat{n} \times \vec{S}_1 \cdot \vec{v}_2 \left( \hat{n} \cdot \vec{v}_2 \right)^2 \vec{v}_1 \cdot \vec{v}_1 - \\ & \left. 2 \vec{S}_1 \times \vec{v}_1 \cdot \vec{v}_2 \hat{n} \cdot \vec{v}_2 \vec{v}_1 \cdot \vec{v}_2 - \frac{1}{2} \hat{n} \times \vec{S}_1 \cdot \vec{v}_2 \vec{v}_1 \cdot \vec{v}_1 \vec{v}_1 \cdot \vec{v}_2 + \frac{1}{2} \hat{n} \times \vec{S}_1 \cdot \vec{v}_2 \vec{v}_1 \cdot \vec{v}_1 \vec{v}_2 \cdot \vec{v}_2 \right) m_1 m_2 G^2 \} \end{aligned}$$

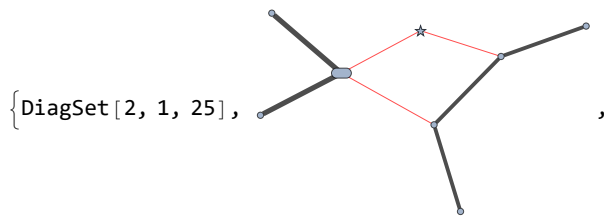

$$\frac{1}{r^2} G^2 m_2^2 \left( 4 (\hat{n} \cdot \vec{v}_2)^2 \vec{S}_1 \times \vec{v}_1 \cdot \vec{a}_1 - 8 \hat{n} \cdot \vec{v}_1 \hat{n} \cdot \vec{v}_2 \vec{S}_1 \times \vec{v}_1 \cdot \vec{a}_1 + 8 \vec{v}_1 \cdot \vec{a}_1 \hat{n} \cdot \vec{v}_2 \hat{n} \times \vec{S}_1 \cdot \vec{v}_1 + 4 \vec{v}_1 \cdot \vec{v}_1 \hat{n} \cdot \vec{v}_2 \hat{n} \times \vec{S}_1 \cdot \vec{a}_1 - \right. \\ \left. 4 \vec{v}_1 \cdot \vec{a}_1 \vec{S}_1 \times \vec{v}_1 \cdot \vec{v}_2 - 2 \vec{v}_1 \cdot \vec{v}_1 \vec{S}_1 \times \vec{a}_1 \cdot \vec{v}_2 + 4 \vec{v}_1 \cdot \vec{v}_2 \vec{S}_1 \times \vec{v}_1 \cdot \vec{a}_1 + 4 \vec{v}_1 \cdot \vec{v}_1 \hat{n} \cdot \vec{v}_2 \hat{n} \times \vec{S}_1 \cdot \vec{v}_1 - 2 \vec{v}_1 \cdot \vec{v}_1 \vec{S}_1 \times \vec{v}_1 \cdot \vec{v}_2 \right) + \\ \frac{G^2 m_2^2 \left( 4 \hat{n} \cdot \vec{v}_2 \vec{S}_1 \times \vec{v}_1 \cdot \vec{a}_1 + 4 \hat{n} \cdot \vec{v}_2 \vec{S}_1 \times \vec{v}_1 \cdot \vec{a}_1 \right)}{r} + \frac{1}{r^3} G^2 m_2^2 \left( 8 \vec{v}_1 \cdot \vec{v}_1 (\hat{n} \cdot \vec{v}_2)^2 \hat{n} \times \vec{S}_1 \cdot \vec{v}_1 - 4 \vec{v}_1 \cdot \vec{v}_1 \hat{n} \cdot \vec{v}_2 \vec{S}_1 \times \vec{v}_1 \cdot \vec{v}_2 - \right. \\ \left. 16 \vec{v}_1 \cdot \vec{v}_1 \hat{n} \cdot \vec{v}_1 \hat{n} \cdot \vec{v}_2 \hat{n} \times \vec{S}_1 \cdot \vec{v}_1 + 4 \vec{v}_1 \cdot \vec{v}_1 \hat{n} \cdot \vec{v}_1 \vec{S}_1 \times \vec{v}_1 \cdot \vec{v}_2 + 4 \vec{v}_1 \cdot \vec{v}_1 \vec{v}_1 \cdot \vec{v}_2 \hat{n} \times \vec{S}_1 \cdot \vec{v}_1 \right) \Big\}$$

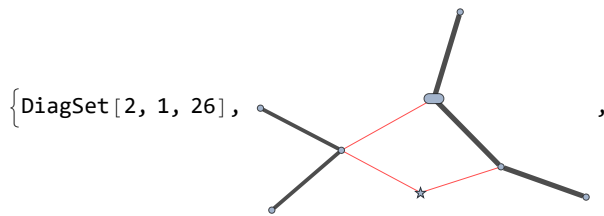

$$\frac{1}{r^2} G^2 m_1 m_2 \left( (\hat{n} \cdot \vec{v}_1)^2 \left( -(\vec{a}_1 \times \vec{S}_1 \cdot \vec{v}_1) \right) + 2 \hat{n} \cdot \vec{v}_2 \hat{n} \cdot \vec{v}_1 \vec{a}_1 \times \vec{S}_1 \cdot \vec{v}_1 - 8 \vec{a}_1 \cdot \vec{v}_1 \hat{n} \cdot \vec{v}_1 \hat{n} \times \vec{S}_1 \cdot \vec{v}_1 - \right. \\ \left. 9 \vec{a}_2 \cdot \vec{v}_2 \hat{n} \cdot \vec{v}_1 \hat{n} \times \vec{S}_1 \cdot \vec{v}_1 - 2 \vec{v}_1 \cdot \vec{v}_1 \hat{n} \cdot \vec{v}_1 \hat{n} \times \vec{a}_1 \cdot \vec{S}_1 + \frac{9}{2} \vec{v}_2 \cdot \vec{v}_2 \hat{n} \cdot \vec{v}_1 \hat{n} \times \vec{a}_1 \cdot \vec{S}_1 + 6 \vec{a}_1 \cdot \vec{v}_1 \hat{n} \cdot \vec{v}_2 \hat{n} \times \vec{S}_1 \cdot \vec{v}_1 - \right. \\ \left. 3 \vec{a}_1 \cdot \vec{v}_1 \vec{S}_1 \times \vec{v}_1 \cdot \vec{v}_2 - \vec{v}_1 \cdot \vec{v}_2 \vec{a}_1 \times \vec{S}_1 \cdot \vec{v}_1 + 2 \vec{v}_1 \cdot \vec{v}_1 \hat{n} \cdot \vec{v}_1 \hat{n} \times \vec{S}_1 \cdot \vec{v}_1 - \frac{9}{2} \vec{v}_2 \cdot \vec{v}_2 \hat{n} \cdot \vec{v}_1 \hat{n} \times \vec{S}_1 \cdot \vec{v}_1 \right) + \\ \frac{1}{r} G^2 m_1 m_2 \left( \hat{n} \cdot \vec{v}_1 \vec{a}_1 \times \vec{S}_1 \cdot \vec{v}_1 + \hat{n} \cdot \vec{v}_1 \vec{a}_1 \times \vec{S}_1 \cdot \vec{v}_1 + 3 \vec{a}_1 \cdot \vec{v}_1 \hat{n} \times \vec{S}_1 \cdot \vec{v}_1 - 3 \vec{a}_1 \cdot \vec{v}_1 \hat{n} \times \vec{a}_1 \cdot \vec{S}_1 \right) + \frac{1}{r^3} \\ G^2 m_1 m_2 \left( -6 \vec{v}_1 \cdot \vec{v}_1 (\hat{n} \cdot \vec{v}_1)^2 \hat{n} \times \vec{S}_1 \cdot \vec{v}_1 + \frac{27}{2} \vec{v}_2 \cdot \vec{v}_2 (\hat{n} \cdot \vec{v}_1)^2 \hat{n} \times \vec{S}_1 \cdot \vec{v}_1 - \right. \\ \left. 2 \vec{v}_1 \cdot \vec{v}_1 \hat{n} \cdot \vec{v}_1 \vec{S}_1 \times \vec{v}_1 \cdot \vec{v}_2 + 8 \vec{v}_1 \cdot \vec{v}_1 \hat{n} \cdot \vec{v}_2 \hat{n} \cdot \vec{v}_1 \hat{n} \times \vec{S}_1 \cdot \vec{v}_1 + \frac{9}{2} \vec{v}_2 \cdot \vec{v}_2 \hat{n} \cdot \vec{v}_1 \vec{S}_1 \times \vec{v}_1 \cdot \vec{v}_2 - \right. \\ \left. 18 \vec{v}_2 \cdot \vec{v}_2 \hat{n} \cdot \vec{v}_2 \hat{n} \cdot \vec{v}_1 \hat{n} \times \vec{S}_1 \cdot \vec{v}_1 - 2 \vec{v}_1 \cdot \vec{v}_1 \vec{v}_1 \cdot \vec{v}_2 \hat{n} \times \vec{S}_1 \cdot \vec{v}_1 + \frac{9}{2} \vec{v}_1 \cdot \vec{v}_2 \vec{v}_2 \cdot \vec{v}_2 \hat{n} \times \vec{S}_1 \cdot \vec{v}_1 \right) \Big\}$$

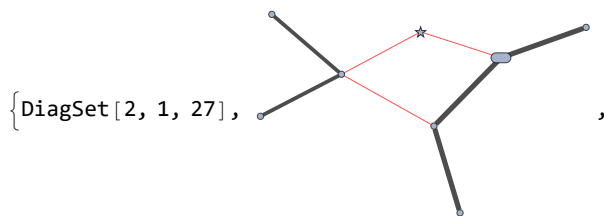

$$\frac{1}{r} \left( -\left( \frac{1}{\vec{a}_1 \times \vec{S}_1 \cdot \vec{v}_1} \right) \hat{n} \cdot \vec{v}_1 - \vec{a}_1 \times \vec{S}_1 \cdot \vec{v}_1 \hat{n} \cdot \vec{v}_1 - 3 \hat{n} \times \vec{S}_1 \cdot \vec{v}_1 \vec{a}_1 \cdot \vec{v}_1 + \right. \\ \left. 3 \hat{n} \times \vec{a}_1 \cdot \vec{S}_1 \vec{a}_1 \cdot \vec{v}_1 + 9 \hat{n} \times \vec{S}_1 \cdot \vec{v}_1 \vec{a}_2 \cdot \vec{v}_2 - 9 \hat{n} \times \vec{a}_1 \cdot \vec{S}_1 \vec{a}_2 \cdot \vec{v}_2 \right) m_1 m_2 G^2 + \frac{1}{r^2} \\ \left( -\left( \vec{a}_1 \times \vec{S}_1 \cdot \vec{v}_1 \right) (\hat{n} \cdot \vec{v}_1)^2 + 2 \vec{a}_1 \times \vec{S}_1 \cdot \vec{v}_1 \hat{n} \cdot \vec{v}_2 \hat{n} \cdot \vec{v}_1 + 4 \hat{n} \times \vec{S}_1 \cdot \vec{v}_1 \vec{a}_1 \cdot \vec{v}_1 \hat{n} \cdot \vec{v}_1 - 9 \hat{n} \times \vec{S}_1 \cdot \vec{v}_1 \vec{a}_2 \cdot \vec{v}_2 \hat{n} \cdot \vec{v}_1 + \right.$$

$$\{\text{DiagSet}[2, 1, 28],$$

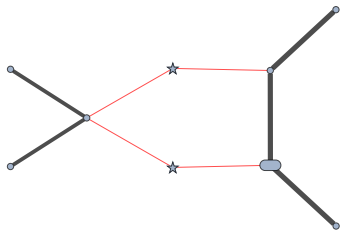

Printed by Wolfram Mathematica Student Edition

$$\begin{aligned} & \vec{a}_1 \times \vec{S}_1 \cdot \vec{v}_2 \vec{v}_1 \cdot \vec{v}_2 + \hat{n} \times \vec{S}_1 \cdot \vec{v}_1 \hat{n} \cdot \vec{a}_1 \vec{v}_1 \cdot \vec{v}_2 - 2 \hat{n} \times \vec{S}_1 \cdot \vec{v}_1 \hat{n} \cdot \vec{v}_2 \vec{v}_1 \cdot \vec{v}_2 + 2 \hat{n} \times \vec{a}_1 \cdot \vec{S}_1 \hat{n} \cdot \vec{v}_2 \vec{v}_1 \cdot \vec{v}_2 \left( m_1 m_2 G^2 + \frac{1}{r^3} \right. \\ & \left. - \frac{3}{2} \hat{n} \times \vec{S}_1 \cdot \vec{v}_1 (\hat{n} \cdot \vec{v}_1)^4 - 2 \vec{S}_1 \times \vec{v}_1 \cdot \vec{v}_2 (\hat{n} \cdot \vec{v}_1)^3 + 12 \hat{n} \times \vec{S}_1 \cdot \vec{v}_1 \hat{n} \cdot \vec{v}_2 (\hat{n} \cdot \vec{v}_1)^3 - 12 \hat{n} \times \vec{S}_1 \cdot \vec{v}_1 (\hat{n} \cdot \vec{v}_2)^2 (\hat{n} \cdot \vec{v}_1)^2 + \right. \\ & 4 \vec{S}_1 \times \vec{v}_1 \cdot \vec{v}_2 \hat{n} \cdot \vec{v}_2 (\hat{n} \cdot \vec{v}_1)^2 + 2 \hat{n} \times \vec{S}_1 \cdot \vec{v}_1 \vec{v}_1 \cdot \vec{v}_1 (\hat{n} \cdot \vec{v}_1)^2 - 6 \hat{n} \times \vec{S}_1 \cdot \vec{v}_1 \vec{v}_1 \cdot \vec{v}_2 (\hat{n} \cdot \vec{v}_1)^2 + \\ & 2 \hat{n} \times \vec{S}_1 \cdot \vec{v}_1 \vec{v}_2 \cdot \vec{v}_2 (\hat{n} \cdot \vec{v}_1)^2 + \vec{S}_1 \times \vec{v}_1 \cdot \vec{v}_2 \vec{v}_1 \cdot \vec{v}_1 \hat{n} \cdot \vec{v}_1 - 4 \hat{n} \times \vec{S}_1 \cdot \vec{v}_1 \hat{n} \cdot \vec{v}_2 \vec{v}_1 \cdot \vec{v}_1 \hat{n} \cdot \vec{v}_1 - 2 \vec{S}_1 \times \vec{v}_1 \cdot \vec{v}_2 \vec{v}_1 \cdot \vec{v}_2 \hat{n} \cdot \vec{v}_1 + \\ & \left. 8 \hat{n} \times \vec{S}_1 \cdot \vec{v}_1 \hat{n} \cdot \vec{v}_2 \vec{v}_1 \cdot \vec{v}_2 \hat{n} \cdot \vec{v}_1 - \frac{1}{2} \hat{n} \times \vec{S}_1 \cdot \vec{v}_1 (\vec{v}_1 \cdot \vec{v}_1)^2 - \hat{n} \times \vec{S}_1 \cdot \vec{v}_1 (\vec{v}_1 \cdot \vec{v}_2)^2 + \hat{n} \times \vec{S}_1 \cdot \vec{v}_1 \vec{v}_1 \cdot \vec{v}_1 \vec{v}_1 \cdot \vec{v}_2 \right) m_1 m_2 G^2 \} \end{aligned}$$

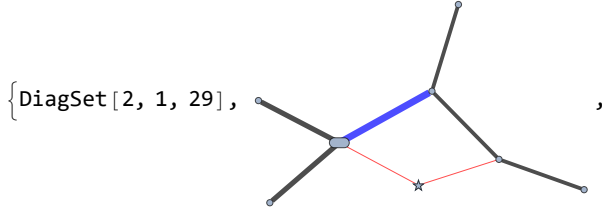

$$\begin{aligned} & \frac{1}{r^2} G^2 m_2^2 \left( -2 (\hat{n} \cdot \vec{v}_2)^2 \vec{S}_1 \times \vec{a}_1 \cdot \vec{v}_2 - 2 (\hat{n} \cdot \vec{v}_2)^2 \vec{S}_1 \times \vec{v}_1 \cdot \vec{a}_2 - 2 \hat{n} \cdot \vec{a}_2 \hat{n} \cdot \vec{v}_2 \vec{S}_1 \times \vec{v}_1 \cdot \vec{v}_2 + 2 \vec{a}_1 \cdot \vec{v}_2 \hat{n} \cdot \vec{v}_2 \hat{n} \times \vec{S}_1 \cdot \vec{v}_2 + \right. \\ & 2 \vec{v}_1 \cdot \vec{a}_2 \hat{n} \cdot \vec{v}_2 \hat{n} \times \vec{S}_1 \cdot \vec{v}_2 + 2 \vec{v}_1 \cdot \vec{v}_2 \hat{n} \cdot \vec{v}_2 \hat{n} \times \vec{S}_1 \cdot \vec{a}_2 + 2 \vec{v}_1 \cdot \vec{v}_2 \vec{S}_1 \times \vec{v}_2 \cdot \vec{a}_2 + 2 \vec{v}_2 \cdot \vec{a}_2 \vec{S}_1 \times \vec{v}_1 \cdot \vec{v}_2 + 2 \vec{v}_2 \cdot \vec{v}_2 \vec{S}_1 \times \vec{a}_1 \cdot \vec{v}_2 + \\ & \left. 2 \vec{v}_2 \cdot \vec{v}_2 \vec{S}_1 \times \vec{v}_1 \cdot \vec{a}_2 - 2 (\hat{n} \cdot \vec{v}_2)^2 \vec{S}_1 \times \vec{v}_1 \cdot \vec{v}_2 + 2 \vec{v}_1 \cdot \vec{v}_2 \hat{n} \cdot \vec{v}_2 \hat{n} \times \vec{S}_1 \cdot \vec{v}_2 + 2 \vec{v}_2 \cdot \vec{v}_2 \vec{S}_1 \times \vec{v}_1 \cdot \vec{v}_2 \right) + \frac{1}{r^3} \\ & G^2 m_2^2 \left( -2 (\hat{n} \cdot \vec{v}_2)^3 \vec{S}_1 \times \vec{v}_1 \cdot \vec{v}_2 + 8 \hat{n} \cdot \vec{v}_1 (\hat{n} \cdot \vec{v}_2)^2 \vec{S}_1 \times \vec{v}_1 \cdot \vec{v}_2 + 2 \vec{v}_1 \cdot \vec{v}_2 (\hat{n} \cdot \vec{v}_2)^2 \hat{n} \times \vec{S}_1 \cdot \vec{v}_2 - 6 \vec{v}_1 \cdot \vec{v}_2 \hat{n} \cdot \vec{v}_2 \vec{S}_1 \times \vec{v}_1 \cdot \vec{v}_2 - \right. \\ & \left. 8 \vec{v}_1 \cdot \vec{v}_2 \hat{n} \cdot \vec{v}_1 \hat{n} \cdot \vec{v}_2 \hat{n} \times \vec{S}_1 \cdot \vec{v}_2 + 2 \vec{v}_2 \cdot \vec{v}_2 \hat{n} \cdot \vec{v}_2 \vec{S}_1 \times \vec{v}_1 \cdot \vec{v}_2 + 2 (\vec{v}_1 \cdot \vec{v}_2)^2 \hat{n} \times \vec{S}_1 \cdot \vec{v}_2 - 4 \vec{v}_2 \cdot \vec{v}_2 \hat{n} \cdot \vec{v}_1 \vec{S}_1 \times \vec{v}_1 \cdot \vec{v}_2 \right) \} \end{aligned}$$

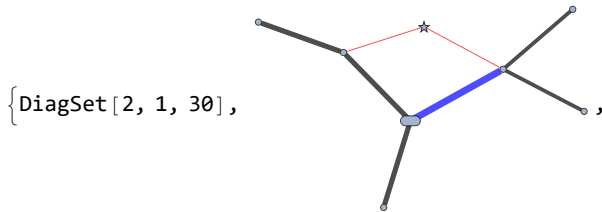

$$\begin{aligned} & \frac{1}{r^2} G^2 m_1 m_2 \left( -3 \vec{a}_1 \cdot \vec{v}_2 \hat{n} \cdot \vec{v}_1 \hat{n} \times \vec{S}_1 \cdot \vec{v}_2 - 3 \vec{a}_2 \cdot \vec{v}_1 \hat{n} \cdot \vec{v}_1 \hat{n} \times \vec{S}_1 \cdot \vec{v}_2 + 6 \vec{a}_2 \cdot \vec{v}_2 \hat{n} \cdot \vec{v}_1 \hat{n} \times \vec{S}_1 \cdot \vec{v}_1 + \right. \\ & 3 \vec{v}_1 \cdot \vec{v}_2 \hat{n} \cdot \vec{v}_1 \hat{n} \times \vec{a}_2 \cdot \vec{S}_1 - 3 \vec{v}_2 \cdot \vec{v}_2 \hat{n} \cdot \vec{v}_1 \hat{n} \times \vec{a}_1 \cdot \vec{S}_1 - 3 \vec{v}_1 \cdot \vec{v}_2 \hat{n} \cdot \vec{v}_1 \hat{n} \times \vec{S}_1 \cdot \vec{v}_2 + 3 \vec{v}_2 \cdot \vec{v}_2 \hat{n} \cdot \vec{v}_1 \hat{n} \times \vec{S}_1 \cdot \vec{v}_1 \left. \right) + \\ & \frac{1}{r^3} G^2 m_1 m_2 \left( 9 \vec{v}_1 \cdot \vec{v}_2 (\hat{n} \cdot \vec{v}_1)^2 \hat{n} \times \vec{S}_1 \cdot \vec{v}_2 - 9 \vec{v}_2 \cdot \vec{v}_2 (\hat{n} \cdot \vec{v}_1)^2 \hat{n} \times \vec{S}_1 \cdot \vec{v}_1 + 3 \vec{v}_1 \cdot \vec{v}_2 \hat{n} \cdot \vec{v}_1 \vec{S}_1 \times \vec{v}_1 \cdot \vec{v}_2 - \right. \\ & 12 \vec{v}_1 \cdot \vec{v}_2 \hat{n} \cdot \vec{v}_2 \hat{n} \cdot \vec{v}_1 \hat{n} \times \vec{S}_1 \cdot \vec{v}_2 - 3 \vec{v}_2 \cdot \vec{v}_2 \hat{n} \cdot \vec{v}_1 \vec{S}_1 \times \vec{v}_1 \cdot \vec{v}_2 + \\ & \left. 12 \vec{v}_2 \cdot \vec{v}_2 \hat{n} \cdot \vec{v}_2 \hat{n} \cdot \vec{v}_1 \hat{n} \times \vec{S}_1 \cdot \vec{v}_1 + 3 (\vec{v}_1 \cdot \vec{v}_2)^2 \hat{n} \times \vec{S}_1 \cdot \vec{v}_2 - 3 \vec{v}_1 \cdot \vec{v}_2 \vec{v}_2 \cdot \vec{v}_2 \hat{n} \times \vec{S}_1 \cdot \vec{v}_1 \right) \} \end{aligned}$$

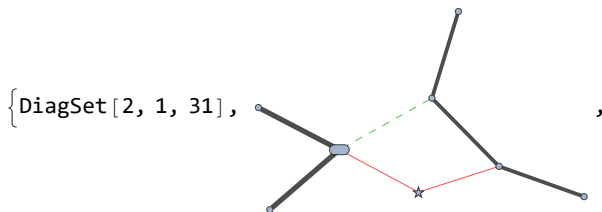

$$\begin{aligned} & \frac{1}{r} G^2 \left( 4 \vec{S}_1 \times \vec{v}_1 \cdot \vec{v}_2 \hat{n} \cdot \vec{a}_2 + 4 \vec{S}_1 \times \vec{a}_1 \cdot \vec{v}_2 \hat{n} \cdot \vec{a}_2 + 4 \vec{S}_1 \times \vec{v}_1 \cdot \vec{a}_2 \hat{n} \cdot \vec{a}_2 - 12 \hat{n} \times \vec{S}_1 \cdot \vec{v}_2 \vec{v}_2 \cdot \vec{a}_2 - 12 \hat{n} \times \vec{S}_1 \cdot \vec{a}_2 \vec{v}_2 \cdot \vec{a}_2 \right) m_2^2 + \\ & \frac{1}{r^2} G^2 \left( 4 \vec{S}_1 \times \vec{v}_1 \cdot \vec{v}_2 (\hat{n} \cdot \vec{v}_2)^2 + 4 \vec{S}_1 \times \vec{a}_1 \cdot \vec{v}_2 (\hat{n} \cdot \vec{v}_2)^2 + 4 \vec{S}_1 \times \vec{v}_1 \cdot \vec{a}_2 (\hat{n} \cdot \vec{v}_2)^2 + \right. \\ & 4 \vec{S}_1 \times \vec{v}_1 \cdot \vec{v}_2 \hat{n} \cdot \vec{a}_2 \hat{n} \cdot \vec{v}_2 - 32 \hat{n} \times \vec{S}_1 \cdot \vec{v}_2 \vec{v}_2 \cdot \vec{a}_2 \hat{n} \cdot \vec{v}_2 + 8 \hat{n} \times \vec{S}_1 \cdot \vec{v}_2 \vec{v}_2 \cdot \vec{v}_2 \hat{n} \cdot \vec{v}_2 + \end{aligned}$$

$$\begin{aligned}
& 8 \hat{n} \times \vec{S}_1 \cdot \vec{a}_2 \vec{v}_2 \cdot \vec{v}_2 \hat{n} \cdot \vec{v}_2 - 8 \vec{S}_1 \times \vec{v}_1 \cdot \vec{v}_2 \hat{n} \cdot \vec{a}_2 \hat{n} \cdot \vec{v}_1 + 4 \vec{S}_1 \times \vec{v}_1 \cdot \vec{v}_2 \vec{v}_1 \cdot \vec{a}_2 + 12 \vec{S}_1 \times \vec{v}_1 \cdot \vec{v}_2 \vec{v}_2 \cdot \vec{a}_2 + \\
& 24 \hat{n} \times \vec{S}_1 \cdot \vec{v}_2 \hat{n} \cdot \vec{v}_1 \vec{v}_2 \cdot \vec{a}_2 - 4 \vec{S}_1 \times \vec{v}_1 \cdot \vec{v}_2 \vec{v}_2 \cdot \vec{v}_2 - 4 \vec{S}_1 \times \vec{a}_1 \cdot \vec{v}_2 \vec{v}_2 \cdot \vec{v}_2 - 4 \vec{S}_1 \times \vec{v}_1 \cdot \vec{a}_2 \vec{v}_2 \cdot \vec{v}_2 \Big) m_2^2 + \\
& \frac{1}{r^3} G^2 \left( 4 \vec{S}_1 \times \vec{v}_1 \cdot \vec{v}_2 (\hat{n} \cdot \vec{v}_2)^3 - 16 \vec{S}_1 \times \vec{v}_1 \cdot \vec{v}_2 \hat{n} \cdot \vec{v}_1 (\hat{n} \cdot \vec{v}_2)^2 + 24 \hat{n} \times \vec{S}_1 \cdot \vec{v}_2 \vec{v}_2 \cdot \vec{v}_2 (\hat{n} \cdot \vec{v}_2)^2 + \right. \\
& 8 \vec{S}_1 \times \vec{v}_1 \cdot \vec{v}_2 \vec{v}_1 \cdot \vec{v}_2 \hat{n} \cdot \vec{v}_2 - 12 \vec{S}_1 \times \vec{v}_1 \cdot \vec{v}_2 \vec{v}_2 \cdot \vec{v}_2 \hat{n} \cdot \vec{v}_2 - 32 \hat{n} \times \vec{S}_1 \cdot \vec{v}_2 \hat{n} \cdot \vec{v}_1 \vec{v}_2 \cdot \vec{v}_2 \hat{n} \cdot \vec{v}_2 + \\
& \left. 8 \vec{S}_1 \times \vec{v}_1 \cdot \vec{v}_2 \hat{n} \cdot \vec{v}_1 \vec{v}_2 \cdot \vec{v}_2 + 8 \hat{n} \times \vec{S}_1 \cdot \vec{v}_2 \vec{v}_1 \cdot \vec{v}_2 \vec{v}_2 \cdot \vec{v}_2 \right) m_2^2 \Big\}
\end{aligned}$$

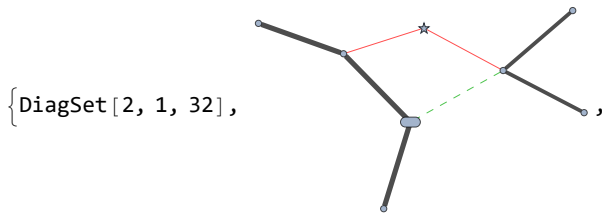

$$\begin{aligned}
& \frac{1}{r} \left( -2 \frac{1}{a_1} \times \vec{S}_1 \cdot \vec{v}_2 \hat{n} \cdot \vec{v}_1 + 2 \vec{S}_1 \times \vec{v}_1 \cdot \vec{v}_2 \hat{n} \cdot \vec{v}_1 - 4 \vec{a}_1 \times \vec{S}_1 \cdot \vec{v}_2 \hat{n} \cdot \vec{v}_1 + \right. \\
& \left. 2 \vec{a}_1 \times \vec{a}_2 \cdot \vec{S}_1 \hat{n} \cdot \vec{v}_1 + 2 \vec{a}_2 \times \vec{S}_1 \cdot \vec{v}_1 \hat{n} \cdot \vec{v}_1 - 3 \hat{n} \times \vec{S}_1 \cdot \vec{v}_2 \vec{a}_1 \cdot \vec{v}_1 + 3 \hat{n} \times \vec{a}_2 \cdot \vec{S}_1 \vec{a}_1 \cdot \vec{v}_1 \right) m_1 m_2 G^2 + \frac{1}{r^2} \\
& \left( -\frac{5}{2} \vec{S}_1 \times \vec{v}_1 \cdot \vec{v}_2 (\hat{n} \cdot \vec{v}_1)^2 + \frac{5}{2} \vec{a}_1 \times \vec{S}_1 \cdot \vec{v}_2 (\hat{n} \cdot \vec{v}_1)^2 - \frac{1}{2} \vec{a}_2 \times \vec{S}_1 \cdot \vec{v}_1 (\hat{n} \cdot \vec{v}_1)^2 - \frac{1}{2} \vec{S}_1 \times \vec{v}_1 \cdot \vec{v}_2 \hat{n} \cdot \vec{a}_1 \hat{n} \cdot \vec{v}_1 + \right. \\
& 4 \vec{S}_1 \times \vec{v}_1 \cdot \vec{v}_2 \hat{n} \cdot \vec{v}_2 \hat{n} \cdot \vec{v}_1 - 4 \vec{a}_1 \times \vec{S}_1 \cdot \vec{v}_2 \hat{n} \cdot \vec{v}_2 \hat{n} \cdot \vec{v}_1 + 9 \hat{n} \times \vec{S}_1 \cdot \vec{v}_2 \vec{a}_1 \cdot \vec{v}_1 \hat{n} \cdot \vec{v}_1 - \frac{3}{2} \hat{n} \times \vec{S}_1 \cdot \vec{v}_1 \vec{a}_1 \cdot \vec{v}_2 \hat{n} \cdot \vec{v}_1 - \\
& \frac{3}{2} \hat{n} \times \vec{S}_1 \cdot \vec{v}_1 \vec{a}_2 \cdot \vec{v}_1 \hat{n} \cdot \vec{v}_1 + 3 \hat{n} \times \vec{S}_1 \cdot \vec{v}_2 \vec{a}_2 \cdot \vec{v}_2 \hat{n} \cdot \vec{v}_1 - \frac{3}{2} \hat{n} \times \vec{S}_1 \cdot \vec{v}_2 \vec{v}_1 \cdot \vec{v}_1 \hat{n} \cdot \vec{v}_1 + \frac{3}{2} \hat{n} \times \vec{a}_2 \cdot \vec{S}_1 \vec{v}_1 \cdot \vec{v}_1 \hat{n} \cdot \vec{v}_1 - \\
& \frac{3}{2} \hat{n} \times \vec{S}_1 \cdot \vec{v}_1 \vec{v}_1 \cdot \vec{v}_2 \hat{n} \cdot \vec{v}_1 + \frac{3}{2} \hat{n} \times \vec{a}_1 \cdot \vec{S}_1 \vec{v}_1 \cdot \vec{v}_2 \hat{n} \cdot \vec{v}_1 + \frac{3}{2} \hat{n} \times \vec{S}_1 \cdot \vec{v}_2 \vec{v}_2 \cdot \vec{v}_2 \hat{n} \cdot \vec{v}_1 - \frac{3}{2} \hat{n} \times \vec{a}_2 \cdot \vec{S}_1 \vec{v}_2 \cdot \vec{v}_2 \hat{n} \cdot \vec{v}_1 + \\
& \left. 3 \vec{S}_1 \times \vec{v}_1 \cdot \vec{v}_2 \vec{a}_1 \cdot \vec{v}_1 - 6 \hat{n} \times \vec{S}_1 \cdot \vec{v}_2 \hat{n} \cdot \vec{v}_2 \vec{a}_1 \cdot \vec{v}_1 - 2 \vec{S}_1 \times \vec{v}_1 \cdot \vec{v}_2 \vec{v}_1 \cdot \vec{v}_2 + 2 \vec{a}_1 \times \vec{S}_1 \cdot \vec{v}_2 \vec{v}_1 \cdot \vec{v}_2 \right) m_1 m_2 G^2 + \frac{1}{r^3} \\
& \left( \frac{3}{2} \vec{S}_1 \times \vec{v}_1 \cdot \vec{v}_2 (\hat{n} \cdot \vec{v}_1)^3 - 2 \vec{S}_1 \times \vec{v}_1 \cdot \vec{v}_2 \hat{n} \cdot \vec{v}_2 (\hat{n} \cdot \vec{v}_1)^2 + \frac{9}{2} \hat{n} \times \vec{S}_1 \cdot \vec{v}_2 \vec{v}_1 \cdot \vec{v}_1 (\hat{n} \cdot \vec{v}_1)^2 + \frac{9}{2} \hat{n} \times \vec{S}_1 \cdot \vec{v}_1 \vec{v}_1 \cdot \vec{v}_2 (\hat{n} \cdot \vec{v}_1)^2 - \right. \\
& \frac{9}{2} \hat{n} \times \vec{S}_1 \cdot \vec{v}_2 \vec{v}_2 \cdot \vec{v}_2 (\hat{n} \cdot \vec{v}_1)^2 + \vec{S}_1 \times \vec{v}_1 \cdot \vec{v}_2 \vec{v}_1 \cdot \vec{v}_1 \hat{n} \cdot \vec{v}_1 - 6 \hat{n} \times \vec{S}_1 \cdot \vec{v}_2 \hat{n} \cdot \vec{v}_2 \vec{v}_1 \cdot \vec{v}_1 \hat{n} \cdot \vec{v}_1 + \frac{5}{2} \vec{S}_1 \times \vec{v}_1 \cdot \vec{v}_2 \vec{v}_1 \cdot \vec{v}_2 \hat{n} \cdot \vec{v}_1 - \\
& 6 \hat{n} \times \vec{S}_1 \cdot \vec{v}_1 \hat{n} \cdot \vec{v}_2 \vec{v}_1 \cdot \vec{v}_2 \hat{n} \cdot \vec{v}_1 - \frac{3}{2} \vec{S}_1 \times \vec{v}_1 \cdot \vec{v}_2 \vec{v}_2 \cdot \vec{v}_2 \hat{n} \cdot \vec{v}_1 + 6 \hat{n} \times \vec{S}_1 \cdot \vec{v}_2 \hat{n} \cdot \vec{v}_2 \vec{v}_2 \cdot \vec{v}_2 \hat{n} \cdot \vec{v}_1 + \\
& \left. \frac{3}{2} \hat{n} \times \vec{S}_1 \cdot \vec{v}_1 (\vec{v}_1 \cdot \vec{v}_2)^2 + \frac{3}{2} \hat{n} \times \vec{S}_1 \cdot \vec{v}_2 \vec{v}_1 \cdot \vec{v}_1 \vec{v}_1 \cdot \vec{v}_2 - \frac{3}{2} \hat{n} \times \vec{S}_1 \cdot \vec{v}_2 \vec{v}_1 \cdot \vec{v}_2 \vec{v}_2 \cdot \vec{v}_2 \right) m_1 m_2 G^2 \Big\}
\end{aligned}$$

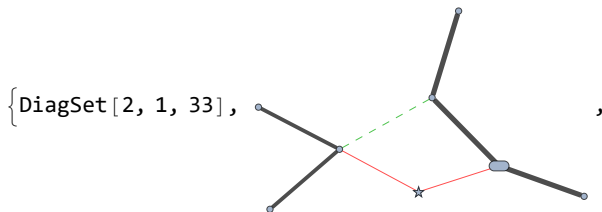

$$\begin{aligned}
& \frac{1}{r^2} G^2 m_1 m_2 \left( -4 \vec{a}_1 \cdot \vec{v}_2 \hat{n} \cdot \vec{v}_1 \hat{n} \times \vec{S}_1 \cdot \vec{v}_1 - 4 \vec{a}_2 \cdot \vec{v}_1 \hat{n} \cdot \vec{v}_1 \hat{n} \times \vec{S}_1 \cdot \vec{v}_1 + 4 \vec{v}_1 \cdot \vec{v}_2 \hat{n} \cdot \vec{v}_1 \hat{n} \times \vec{a}_1 \cdot \vec{S}_1 - 8 \vec{v}_1 \cdot \vec{v}_2 \hat{n} \cdot \vec{v}_2 \hat{n} \times \vec{a}_1 \cdot \vec{S}_1 + \right. \\
& \left. 4 \vec{v}_1 \cdot \vec{v}_2 \vec{a}_1 \times \vec{S}_1 \cdot \vec{v}_2 - 4 \vec{v}_1 \cdot \vec{v}_2 \hat{n} \cdot \vec{v}_1 \hat{n} \times \vec{S}_1 \cdot \vec{v}_1 + 8 \vec{v}_1 \cdot \vec{v}_2 \hat{n} \cdot \vec{v}_2 \hat{n} \times \vec{S}_1 \cdot \vec{v}_1 - 4 \vec{v}_1 \cdot \vec{v}_2 \vec{S}_1 \times \vec{v}_1 \cdot \vec{v}_2 \right) + \frac{1}{r} \\
& G^2 m_1 m_2 \left( 4 \vec{a}_1 \cdot \vec{v}_2 \hat{n} \times \vec{S}_1 \cdot \vec{v}_1 - 4 \vec{a}_1 \cdot \vec{v}_2 \hat{n} \times \vec{a}_1 \cdot \vec{S}_1 + 4 \vec{a}_2 \cdot \vec{v}_1 \hat{n} \times \vec{S}_1 \cdot \vec{v}_1 - 4 \vec{a}_2 \cdot \vec{v}_1 \hat{n} \times \vec{a}_1 \cdot \vec{S}_1 \right) + \frac{1}{r^3} G^2 m_1 m_2 \\
& \left( 4 \vec{v}_1 \cdot \vec{v}_2 (\hat{n} \cdot \vec{v}_1)^2 \hat{n} \times \vec{S}_1 \cdot \vec{v}_1 + 4 \vec{v}_1 \cdot \vec{v}_2 \hat{n} \cdot \vec{v}_1 \vec{S}_1 \times \vec{v}_1 \cdot \vec{v}_2 - 16 \vec{v}_1 \cdot \vec{v}_2 \hat{n} \cdot \vec{v}_2 \hat{n} \cdot \vec{v}_1 \hat{n} \times \vec{S}_1 \cdot \vec{v}_1 + 4 (\vec{v}_1 \cdot \vec{v}_2)^2 \hat{n} \times \vec{S}_1 \cdot \vec{v}_1 \right) \Big\}
\end{aligned}$$

$\{\text{DiagSet}[2, 1, 34],$ 
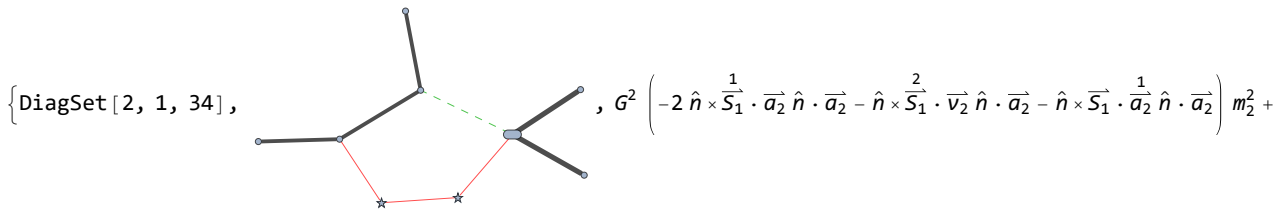
 $, G^2 \left( -2 \hat{n} \times \vec{S}_1 \cdot \vec{a}_2 \hat{n} \cdot \vec{a}_2 - \hat{n} \times \vec{S}_1 \cdot \vec{v}_2 \hat{n} \cdot \vec{a}_2 - \hat{n} \times \vec{S}_1 \cdot \vec{a}_2 \hat{n} \cdot \vec{a}_2 \right) m_2^2 +$

$$\begin{aligned} & \frac{1}{r} G^2 \left( -3 \hat{n} \times \vec{S}_1 \cdot \vec{v}_2 (\hat{n} \cdot \vec{a}_2)^2 + 2 \vec{S}_1 \times \vec{v}_1 \cdot \vec{v}_2 \hat{n} \cdot \vec{a}_2 + \vec{S}_1 \times \vec{a}_1 \cdot \vec{v}_2 \hat{n} \cdot \vec{a}_2 + 2 \vec{S}_1 \times \vec{v}_1 \cdot \vec{a}_2 \hat{n} \cdot \vec{a}_2 - \vec{S}_1 \times \vec{v}_2 \cdot \vec{a}_2 \hat{n} \cdot \vec{a}_2 + \right. \\ & 2 \hat{n} \times \vec{S}_1 \cdot \vec{v}_2 \hat{n} \cdot \vec{a}_1 \hat{n} \cdot \vec{a}_2 + 4 \hat{n} \times \vec{S}_1 \cdot \vec{v}_2 \hat{n} \cdot \vec{v}_1 \hat{n} \cdot \vec{a}_2 + 4 \hat{n} \times \vec{S}_1 \cdot \vec{a}_2 \hat{n} \cdot \vec{v}_1 \hat{n} \cdot \vec{a}_2 - 6 \hat{n} \times \vec{S}_1 \cdot \vec{v}_2 \hat{n} \cdot \vec{v}_2 \hat{n} \cdot \vec{a}_2 - \\ & 6 \hat{n} \times \vec{S}_1 \cdot \vec{a}_2 \hat{n} \cdot \vec{v}_2 \hat{n} \cdot \vec{a}_2 + 2 \hat{n} \times \vec{S}_1 \cdot \vec{a}_2 (\hat{n} \cdot \vec{v}_2)^2 + \hat{n} \times \vec{S}_1 \cdot \vec{v}_2 (\hat{n} \cdot \vec{v}_2)^2 + \hat{n} \times \vec{S}_1 \cdot \vec{a}_2 (\hat{n} \cdot \vec{v}_2)^2 - \hat{n} \times \vec{S}_1 \cdot \vec{v}_2 \vec{a}_1 \cdot \vec{a}_2 - \\ & \left. 2 \hat{n} \times \vec{S}_1 \cdot \vec{v}_2 \vec{v}_1 \cdot \vec{a}_2 - 2 \hat{n} \times \vec{S}_1 \cdot \vec{a}_2 \vec{v}_1 \cdot \vec{a}_2 + 2 \hat{n} \times \vec{S}_1 \cdot \vec{a}_2 \vec{v}_2 \cdot \vec{v}_2 + \hat{n} \times \vec{S}_1 \cdot \vec{v}_2 \vec{v}_2 \cdot \vec{v}_2 + \hat{n} \times \vec{S}_1 \cdot \vec{a}_2 \vec{v}_2 \cdot \vec{v}_2 \right) m_2^2 + \\ & \frac{1}{r^2} G^2 \left( 6 \hat{n} \times \vec{S}_1 \cdot \vec{v}_2 (\hat{n} \cdot \vec{v}_2)^3 + 6 \hat{n} \times \vec{S}_1 \cdot \vec{a}_2 (\hat{n} \cdot \vec{v}_2)^3 - 2 \vec{S}_1 \times \vec{v}_1 \cdot \vec{v}_2 (\hat{n} \cdot \vec{v}_2)^2 - \vec{S}_1 \times \vec{a}_1 \cdot \vec{v}_2 (\hat{n} \cdot \vec{v}_2)^2 - \right. \\ & 2 \vec{S}_1 \times \vec{v}_1 \cdot \vec{a}_2 (\hat{n} \cdot \vec{v}_2)^2 + \vec{S}_1 \times \vec{v}_2 \cdot \vec{a}_2 (\hat{n} \cdot \vec{v}_2)^2 - 4 \hat{n} \times \vec{S}_1 \cdot \vec{v}_2 \hat{n} \cdot \vec{a}_1 (\hat{n} \cdot \vec{v}_2)^2 - 12 \hat{n} \times \vec{S}_1 \cdot \vec{v}_2 \hat{n} \cdot \vec{a}_2 (\hat{n} \cdot \vec{v}_2)^2 - \\ & 8 \hat{n} \times \vec{S}_1 \cdot \vec{v}_2 \hat{n} \cdot \vec{v}_1 (\hat{n} \cdot \vec{v}_2)^2 - 8 \hat{n} \times \vec{S}_1 \cdot \vec{a}_2 \hat{n} \cdot \vec{v}_1 (\hat{n} \cdot \vec{v}_2)^2 + 6 \vec{S}_1 \times \vec{v}_1 \cdot \vec{v}_2 \hat{n} \cdot \vec{a}_2 \hat{n} \cdot \vec{v}_2 + \\ & 24 \hat{n} \times \vec{S}_1 \cdot \vec{v}_2 \hat{n} \cdot \vec{a}_2 \hat{n} \cdot \vec{v}_1 \hat{n} \cdot \vec{v}_2 + 2 \hat{n} \times \vec{S}_1 \cdot \vec{v}_2 \vec{a}_1 \cdot \vec{v}_2 \hat{n} \cdot \vec{v}_2 - 6 \hat{n} \times \vec{S}_1 \cdot \vec{v}_2 \vec{v}_1 \cdot \vec{a}_2 \hat{n} \cdot \vec{v}_2 + 4 \hat{n} \times \vec{S}_1 \cdot \vec{v}_2 \vec{v}_1 \cdot \vec{v}_2 \hat{n} \cdot \vec{v}_2 + \\ & 4 \hat{n} \times \vec{S}_1 \cdot \vec{a}_2 \vec{v}_1 \cdot \vec{v}_2 \hat{n} \cdot \vec{v}_2 + 6 \hat{n} \times \vec{S}_1 \cdot \vec{v}_2 \vec{v}_2 \cdot \vec{v}_2 \hat{n} \cdot \vec{v}_2 + 6 \hat{n} \times \vec{S}_1 \cdot \vec{a}_2 \vec{v}_2 \cdot \vec{v}_2 \hat{n} \cdot \vec{v}_2 - 8 \hat{n} \times \vec{S}_1 \cdot \vec{v}_2 \hat{n} \cdot \vec{a}_2 (\hat{n} \cdot \vec{v}_1)^2 - \\ & 4 \vec{S}_1 \times \vec{v}_1 \cdot \vec{v}_2 \hat{n} \cdot \vec{a}_2 \hat{n} \cdot \vec{v}_1 + 2 \vec{S}_1 \times \vec{v}_1 \cdot \vec{v}_2 \vec{v}_1 \cdot \vec{a}_2 + 4 \hat{n} \times \vec{S}_1 \cdot \vec{v}_2 \hat{n} \cdot \vec{v}_1 \vec{v}_1 \cdot \vec{a}_2 + 2 \hat{n} \times \vec{S}_1 \cdot \vec{v}_2 \hat{n} \cdot \vec{a}_2 \vec{v}_1 \cdot \vec{v}_1 - \\ & 6 \hat{n} \times \vec{S}_1 \cdot \vec{v}_2 \hat{n} \cdot \vec{a}_2 \vec{v}_1 \cdot \vec{v}_2 - 2 \vec{S}_1 \times \vec{v}_1 \cdot \vec{v}_2 \vec{v}_2 \cdot \vec{v}_2 - \vec{S}_1 \times \vec{a}_1 \cdot \vec{v}_2 \vec{v}_2 \cdot \vec{v}_2 - 2 \vec{S}_1 \times \vec{v}_1 \cdot \vec{a}_2 \vec{v}_2 \cdot \vec{v}_2 + \vec{S}_1 \times \vec{v}_2 \cdot \vec{a}_2 \vec{v}_2 \cdot \vec{v}_2 - \\ & \left. 2 \hat{n} \times \vec{S}_1 \cdot \vec{v}_2 \hat{n} \cdot \vec{a}_1 \vec{v}_2 \cdot \vec{v}_2 + 6 \hat{n} \times \vec{S}_1 \cdot \vec{v}_2 \hat{n} \cdot \vec{a}_2 \vec{v}_2 \cdot \vec{v}_2 - 4 \hat{n} \times \vec{S}_1 \cdot \vec{v}_2 \hat{n} \cdot \vec{v}_1 \vec{v}_2 \cdot \vec{v}_2 - 4 \hat{n} \times \vec{S}_1 \cdot \vec{a}_2 \hat{n} \cdot \vec{v}_1 \vec{v}_2 \cdot \vec{v}_2 \right) m_2^2 + \frac{1}{r^3} \\ & G^2 \left( 15 \hat{n} \times \vec{S}_1 \cdot \vec{v}_2 (\hat{n} \cdot \vec{v}_2)^4 - 6 \vec{S}_1 \times \vec{v}_1 \cdot \vec{v}_2 (\hat{n} \cdot \vec{v}_2)^3 - 36 \hat{n} \times \vec{S}_1 \cdot \vec{v}_2 \hat{n} \cdot \vec{v}_1 (\hat{n} \cdot \vec{v}_2)^3 + 24 \hat{n} \times \vec{S}_1 \cdot \vec{v}_2 (\hat{n} \cdot \vec{v}_1)^2 (\hat{n} \cdot \vec{v}_2)^2 + \right. \\ & 8 \vec{S}_1 \times \vec{v}_1 \cdot \vec{v}_2 \hat{n} \cdot \vec{v}_1 (\hat{n} \cdot \vec{v}_2)^2 - 4 \hat{n} \times \vec{S}_1 \cdot \vec{v}_2 \vec{v}_1 \cdot \vec{v}_1 (\hat{n} \cdot \vec{v}_2)^2 + 18 \hat{n} \times \vec{S}_1 \cdot \vec{v}_2 \vec{v}_1 \cdot \vec{v}_2 (\hat{n} \cdot \vec{v}_2)^2 + \\ & 12 \hat{n} \times \vec{S}_1 \cdot \vec{v}_2 \vec{v}_2 \cdot \vec{v}_2 (\hat{n} \cdot \vec{v}_2)^2 - 4 \vec{S}_1 \times \vec{v}_1 \cdot \vec{v}_2 \vec{v}_1 \cdot \vec{v}_2 \hat{n} \cdot \vec{v}_2 - 16 \hat{n} \times \vec{S}_1 \cdot \vec{v}_2 \hat{n} \cdot \vec{v}_1 \vec{v}_1 \cdot \vec{v}_2 \hat{n} \cdot \vec{v}_2 - \\ & 6 \vec{S}_1 \times \vec{v}_1 \cdot \vec{v}_2 \vec{v}_2 \cdot \vec{v}_2 \hat{n} \cdot \vec{v}_2 - 24 \hat{n} \times \vec{S}_1 \cdot \vec{v}_2 \hat{n} \cdot \vec{v}_1 \vec{v}_2 \cdot \vec{v}_2 \hat{n} \cdot \vec{v}_2 + 2 \hat{n} \times \vec{S}_1 \cdot \vec{v}_2 (\vec{v}_1 \cdot \vec{v}_2)^2 - 3 \hat{n} \times \vec{S}_1 \cdot \vec{v}_2 (\vec{v}_2 \cdot \vec{v}_2)^2 + \\ & \left. 8 \hat{n} \times \vec{S}_1 \cdot \vec{v}_2 (\hat{n} \cdot \vec{v}_1)^2 \vec{v}_2 \cdot \vec{v}_2 + 4 \vec{S}_1 \times \vec{v}_1 \cdot \vec{v}_2 \hat{n} \cdot \vec{v}_1 \vec{v}_2 \cdot \vec{v}_2 - 2 \hat{n} \times \vec{S}_1 \cdot \vec{v}_2 \vec{v}_1 \cdot \vec{v}_1 \vec{v}_2 \cdot \vec{v}_2 + 6 \hat{n} \times \vec{S}_1 \cdot \vec{v}_2 \vec{v}_1 \cdot \vec{v}_2 \vec{v}_2 \cdot \vec{v}_2 \right\} m_2^2 \Bigg] \end{aligned}$$

$\{\text{DiagSet}[2, 1, 35],$

$$\begin{aligned} & \left( -\frac{1}{4} \hat{n} \times \vec{a}_2 \cdot \vec{S}_1 \hat{n} \cdot \vec{a}_1 + \frac{1}{4} \hat{n} \times \vec{S}_1 \cdot \vec{v}_2 \hat{n} \cdot \vec{a}_1 - \frac{1}{2} \hat{n} \times \vec{a}_2 \cdot \vec{S}_1 \hat{n} \cdot \vec{a}_1 \right) m_1 m_2 G^2 + \frac{1}{r} \\ & \left( -\frac{3}{4} \hat{n} \times \vec{S}_1 \cdot \vec{v}_2 (\hat{n} \cdot \vec{a}_1)^2 - \frac{1}{2} \vec{S}_1 \times \vec{v}_1 \cdot \vec{v}_2 \hat{n} \cdot \vec{a}_1 + \frac{1}{4} \vec{a}_1 \times \vec{S}_1 \cdot \vec{v}_2 \hat{n} \cdot \vec{a}_1 - \frac{1}{2} \vec{a}_2 \times \vec{S}_1 \cdot \vec{v}_1 \hat{n} \cdot \vec{a}_1 + \frac{1}{4} \vec{a}_2 \times \vec{S}_1 \cdot \vec{v}_2 \hat{n} \cdot \vec{a}_1 + \right. \\ & \quad \frac{1}{2} \hat{n} \times \vec{S}_1 \cdot \vec{v}_2 \hat{n} \cdot \vec{a}_2 \hat{n} \cdot \vec{a}_1 - \frac{3}{2} \hat{n} \times \vec{S}_1 \cdot \vec{v}_2 \hat{n} \cdot \vec{v}_1 \hat{n} \cdot \vec{a}_1 + \frac{3}{2} \hat{n} \times \vec{a}_2 \cdot \vec{S}_1 \hat{n} \cdot \vec{v}_1 \hat{n} \cdot \vec{a}_1 + \hat{n} \times \vec{S}_1 \cdot \vec{v}_2 \hat{n} \cdot \vec{v}_2 \hat{n} \cdot \vec{a}_1 - \\ & \quad \hat{n} \times \vec{a}_2 \cdot \vec{S}_1 \hat{n} \cdot \vec{v}_2 \hat{n} \cdot \vec{a}_1 - \frac{1}{4} \hat{n} \times \vec{a}_2 \cdot \vec{S}_1 (\hat{n} \cdot \vec{v}_1)^2 + \frac{1}{4} \hat{n} \times \vec{S}_1 \cdot \vec{v}_2 (\hat{n} \cdot \vec{v}_1)^2 - \frac{1}{2} \hat{n} \times \vec{a}_2 \cdot \vec{S}_1 (\hat{n} \cdot \vec{v}_1)^2 - \frac{1}{4} \hat{n} \times \vec{S}_1 \cdot \vec{v}_2 \vec{a}_1 \cdot \vec{a}_2 - \\ & \quad \left. \frac{1}{2} \hat{n} \times \vec{S}_1 \cdot \vec{v}_2 \vec{a}_1 \cdot \vec{v}_2 + \frac{1}{2} \hat{n} \times \vec{a}_2 \cdot \vec{S}_1 \vec{a}_1 \cdot \vec{v}_2 - \frac{1}{4} \hat{n} \times \vec{a}_2 \cdot \vec{S}_1 \vec{v}_1 \cdot \vec{v}_1 + \frac{1}{4} \hat{n} \times \vec{S}_1 \cdot \vec{v}_2 \vec{v}_1 \cdot \vec{v}_1 - \frac{1}{2} \hat{n} \times \vec{a}_2 \cdot \vec{S}_1 \vec{v}_1 \cdot \vec{v}_1 \right) m_1 m_2 G^2 + \\ & \frac{1}{r^2} \left( -\frac{3}{2} \hat{n} \times \vec{S}_1 \cdot \vec{v}_2 (\hat{n} \cdot \vec{v}_1)^3 + \frac{3}{2} \hat{n} \times \vec{a}_2 \cdot \vec{S}_1 (\hat{n} \cdot \vec{v}_1)^3 - \frac{1}{2} \vec{S}_1 \times \vec{v}_1 \cdot \vec{v}_2 (\hat{n} \cdot \vec{v}_1)^2 + \frac{1}{4} \vec{a}_1 \times \vec{S}_1 \cdot \vec{v}_2 (\hat{n} \cdot \vec{v}_1)^2 - \right. \end{aligned}$$





$$2 \vec{S_1} \times \vec{v_2} \cdot \vec{a_2} \vec{v_2} \cdot \vec{v_2} - 4 \hat{n} \times \vec{S_1} \cdot \vec{v_2} \hat{n} \cdot \vec{a_2} \vec{v_2} \cdot \vec{v_2} + 4 \hat{n} \times \vec{S_1} \cdot \vec{a_2} \hat{n} \cdot \vec{v_1} \vec{v_2} \cdot \vec{v_2} \Big) m_2^2 + \frac{1}{r^3} \\ G^2 \Big\{ 6 \hat{n} \times \vec{S_1} \cdot \vec{v_2} (\hat{n} \cdot \vec{v_2})^4 - 8 \vec{S_1} \times \vec{v_1} \cdot \vec{v_2} (\hat{n} \cdot \vec{v_2})^3 - 48 \hat{n} \times \vec{S_1} \cdot \vec{v_2} \hat{n} \cdot \vec{v_1} (\hat{n} \cdot \vec{v_2})^3 + 48 \hat{n} \times \vec{S_1} \cdot \vec{v_2} (\hat{n} \cdot \vec{v_1})^2 (\hat{n} \cdot \vec{v_2})^2 + \\ 16 \vec{S_1} \times \vec{v_1} \cdot \vec{v_2} \hat{n} \cdot \vec{v_1} (\hat{n} \cdot \vec{v_2})^2 - 8 \hat{n} \times \vec{S_1} \cdot \vec{v_2} \vec{v_1} \cdot \vec{v_1} (\hat{n} \cdot \vec{v_2})^2 + 24 \hat{n} \times \vec{S_1} \cdot \vec{v_2} \vec{v_1} \cdot \vec{v_2} (\hat{n} \cdot \vec{v_2})^2 - 8 \hat{n} \times \vec{S_1} \cdot \vec{v_2} \\ \vec{v_2} \cdot \vec{v_2} (\hat{n} \cdot \vec{v_2})^2 - 8 \vec{S_1} \times \vec{v_1} \cdot \vec{v_2} \vec{v_1} \cdot \vec{v_2} \hat{n} \cdot \vec{v_2} - 32 \hat{n} \times \vec{S_1} \cdot \vec{v_2} \hat{n} \cdot \vec{v_1} \vec{v_1} \cdot \vec{v_2} \hat{n} \cdot \vec{v_2} + 4 \vec{S_1} \times \vec{v_1} \cdot \vec{v_2} \vec{v_2} \cdot \vec{v_2} \hat{n} \cdot \vec{v_2} + \\ 16 \hat{n} \times \vec{S_1} \cdot \vec{v_2} \hat{n} \cdot \vec{v_1} \vec{v_2} \cdot \vec{v_2} \hat{n} \cdot \vec{v_2} + 4 \hat{n} \times \vec{S_1} \cdot \vec{v_2} (\vec{v_1} \cdot \vec{v_2})^2 + 2 \hat{n} \times \vec{S_1} \cdot \vec{v_2} (\vec{v_2} \cdot \vec{v_2})^2 - 4 \hat{n} \times \vec{S_1} \cdot \vec{v_2} \vec{v_1} \cdot \vec{v_2} \vec{v_2} \cdot \vec{v_2} \Big\} m_2^2$$

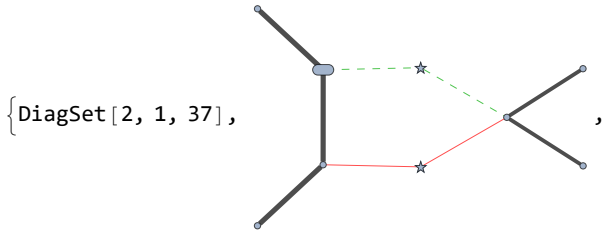

[illegible]

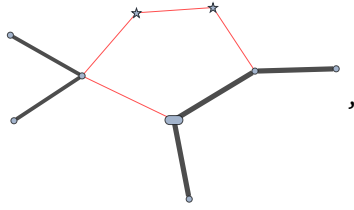

$$\{\text{DiagSet}[2, 1, 39],$$

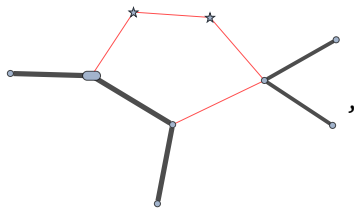

$$\left(-\frac{1}{4}\vec{a_1} \times \vec{a_2} \cdot \vec{S_1} - \frac{1}{2}\vec{a_1} \times \vec{a_2} \cdot \vec{S_1} - \frac{1}{4}\vec{a_2} \times \vec{S_1} \cdot \vec{v_1} + \frac{1}{4}\hat{n} \times \vec{a_1} \cdot \vec{S_1} \hat{n} \cdot \vec{a_1} - \frac{1}{4}\hat{n} \times \vec{S_1} \cdot \vec{v_1} \hat{n} \cdot \vec{a_1} + \frac{1}{2}\hat{n} \times \vec{a_1} \cdot \vec{S_1} \hat{n} \cdot \vec{a_1}\right) m_1 m_2 G^2 +$$

[illegible]

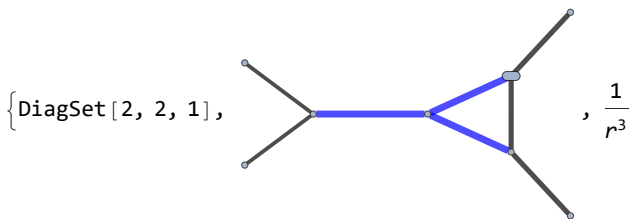

$$G^2 m_1 m_2 \left( -24 \vec{v}_1 \cdot \vec{v}_2 (\hat{n} \cdot \vec{v}_1)^2 \hat{n} \times \vec{S}_1 \cdot \vec{v}_2 + 24 \vec{v}_2 \cdot \vec{v}_2 (\hat{n} \cdot \vec{v}_1)^2 \hat{n} \times \vec{S}_1 \cdot \vec{v}_1 - 10 \vec{v}_1 \cdot \vec{v}_2 \hat{n} \cdot \vec{v}_1 \vec{S}_1 \times \vec{v}_1 \cdot \vec{v}_2 - \right. \\ \left. 7 (\vec{v}_1 \cdot \vec{v}_2)^2 \hat{n} \times \vec{S}_1 \cdot \vec{v}_1 + 2 \vec{v}_1 \cdot \vec{v}_1 \hat{n} \cdot \vec{v}_2 \vec{S}_1 \times \vec{v}_1 \cdot \vec{v}_2 + 4 \vec{v}_1 \cdot \vec{v}_1 \vec{v}_1 \cdot \vec{v}_2 \hat{n} \times \vec{S}_1 \cdot \vec{v}_2 + 3 \vec{v}_1 \cdot \vec{v}_1 \vec{v}_2 \cdot \vec{v}_2 \hat{n} \times \vec{S}_1 \cdot \vec{v}_1 \right) \Big\}$$

$$\left\{ \text{DiagSet}[2, 2, 2], \frac{1}{r^3} \right\}$$

$$G^2 m_2^2 \left( -32 \vec{v}_1 \cdot \vec{v}_2 (\hat{n} \cdot \vec{v}_2)^2 \hat{n} \times \vec{S}_1 \cdot \vec{v}_2 + 32 \vec{v}_2 \cdot \vec{v}_2 (\hat{n} \cdot \vec{v}_2)^2 \hat{n} \times \vec{S}_1 \cdot \vec{v}_1 - 16 \vec{v}_2 \cdot \vec{v}_2 \hat{n} \cdot \vec{v}_2 \vec{S}_1 \times \vec{v}_1 \cdot \vec{v}_2 \right)$$

$$\left\{ \text{DiagSet}[2, 2, 3], \frac{1}{r^2} \right\}$$

$$G^2 m_1 m_2 \left( 20 \vec{a}_1 \cdot \vec{v}_2 \hat{n} \cdot \vec{v}_1 \hat{n} \times \vec{S}_1 \cdot \vec{v}_1 - 16 \vec{v}_1 \cdot \vec{a}_1 \hat{n} \cdot \vec{v}_1 \hat{n} \times \vec{S}_1 \cdot \vec{v}_2 - 4 \vec{v}_1 \cdot \vec{a}_1 \hat{n} \cdot \vec{v}_2 \hat{n} \times \vec{S}_1 \cdot \vec{v}_1 - 4 \vec{v}_1 \cdot \vec{v}_1 \hat{n} \cdot \vec{a}_1 \hat{n} \times \vec{S}_1 \cdot \vec{v}_2 + \right. \\ \left. 4 \vec{v}_1 \cdot \vec{v}_1 \hat{n} \cdot \vec{v}_2 \hat{n} \times \vec{S}_1 \cdot \vec{a}_1 + 4 \vec{v}_1 \cdot \vec{v}_2 \hat{n} \cdot \vec{a}_1 \hat{n} \times \vec{S}_1 \cdot \vec{v}_1 - 4 \vec{v}_1 \cdot \vec{v}_2 \hat{n} \cdot \vec{v}_1 \hat{n} \times \vec{S}_1 \cdot \vec{a}_1 - 4 \vec{v}_1 \cdot \vec{a}_1 \vec{S}_1 \times \vec{v}_1 \cdot \vec{v}_2 - \right. \\ \left. 4 \vec{v}_1 \cdot \vec{v}_2 \vec{S}_1 \times \vec{v}_1 \cdot \vec{a}_1 + 4 \vec{v}_1 \cdot \vec{v}_1 \hat{n} \cdot \vec{v}_1 \hat{n} \times \vec{S}_1 \cdot \vec{v}_2 - 4 \vec{v}_1 \cdot \vec{v}_2 \hat{n} \cdot \vec{v}_1 \hat{n} \times \vec{S}_1 \cdot \vec{v}_1 + 4 \vec{v}_1 \cdot \vec{v}_1 \vec{S}_1 \times \vec{v}_1 \cdot \vec{v}_2 \right)$$

$$\left\{ \text{DiagSet}[2, 2, 4], \right\}$$

$$\frac{1}{r^2} \left( -2 \vec{S}_1 \times \vec{v}_1 \cdot \vec{v}_2 \vec{a}_1 \cdot \vec{v}_2 - 8 \hat{n} \times \vec{S}_1 \cdot \vec{v}_2 \hat{n} \cdot \vec{v}_1 \vec{a}_1 \cdot \vec{v}_2 - 6 \hat{n} \times \vec{S}_1 \cdot \vec{v}_1 \hat{n} \cdot \vec{v}_2 \vec{a}_1 \cdot \vec{v}_2 - 12 \hat{n} \times \vec{S}_1 \cdot \vec{v}_2 \hat{n} \cdot \vec{v}_2 \vec{v}_1 \cdot \vec{a}_1 + \right. \\ \left. 12 \hat{n} \times \vec{S}_1 \cdot \vec{v}_2 \hat{n} \cdot \vec{v}_1 \vec{v}_1 \cdot \vec{a}_2 + 8 \hat{n} \times \vec{S}_1 \cdot \vec{v}_1 \hat{n} \cdot \vec{v}_2 \vec{v}_1 \cdot \vec{a}_2 - 8 \hat{n} \times \vec{S}_1 \cdot \vec{v}_2 \hat{n} \cdot \vec{a}_2 \vec{v}_1 \cdot \vec{v}_1 - 10 \hat{n} \times \vec{S}_1 \cdot \vec{v}_2 \hat{n} \cdot \vec{v}_2 \vec{v}_1 \cdot \vec{v}_1 - \right. \\ \left. 8 \hat{n} \times \vec{S}_1 \cdot \vec{a}_2 \hat{n} \cdot \vec{v}_2 \vec{v}_1 \cdot \vec{v}_1 - 6 \vec{S}_1 \times \vec{v}_1 \cdot \vec{v}_2 \vec{v}_1 \cdot \vec{v}_2 - 6 \vec{S}_1 \times \vec{a}_1 \cdot \vec{v}_2 \vec{v}_1 \cdot \vec{v}_2 + 8 \hat{n} \times \vec{S}_1 \cdot \vec{v}_2 \hat{n} \cdot \vec{a}_1 \vec{v}_1 \cdot \vec{v}_2 + \right. \\ \left. 8 \hat{n} \times \vec{S}_1 \cdot \vec{v}_1 \hat{n} \cdot \vec{a}_2 \vec{v}_1 \cdot \vec{v}_2 + 12 \hat{n} \times \vec{S}_1 \cdot \vec{a}_2 \hat{n} \cdot \vec{v}_1 \vec{v}_1 \cdot \vec{v}_2 + 10 \hat{n} \times \vec{S}_1 \cdot \vec{v}_1 \hat{n} \cdot \vec{v}_2 \vec{v}_1 \cdot \vec{v}_2 + 18 \hat{n} \times \vec{S}_1 \cdot \vec{a}_1 \hat{n} \cdot \vec{v}_2 \vec{v}_1 \cdot \vec{v}_2 - \right. \\ \left. 24 \hat{n} \times \vec{S}_1 \cdot \vec{v}_1 \hat{n} \cdot \vec{v}_1 \vec{v}_2 \cdot \vec{a}_2 + 8 \vec{S}_1 \times \vec{v}_1 \cdot \vec{a}_1 \vec{v}_2 \cdot \vec{v}_2 - 8 \hat{n} \times \vec{S}_1 \cdot \vec{v}_1 \hat{n} \cdot \vec{a}_1 \vec{v}_2 \cdot \vec{v}_2 + 8 \hat{n} \times \vec{S}_1 \cdot \vec{a}_1 \hat{n} \cdot \vec{v}_1 \vec{v}_2 \cdot \vec{v}_2 \right) m_1 m_2 G^2 + \\ \frac{1}{r^3} \left( -32 \hat{n} \times \vec{S}_1 \cdot \vec{v}_2 \vec{v}_1 \cdot \vec{v}_1 (\hat{n} \cdot \vec{v}_2)^2 + 32 \hat{n} \times \vec{S}_1 \cdot \vec{v}_1 \vec{v}_1 \cdot \vec{v}_2 (\hat{n} \cdot \vec{v}_2)^2 + 6 \vec{S}_1 \times \vec{v}_1 \cdot \vec{v}_2 \vec{v}_1 \cdot \vec{v}_1 \hat{n} \cdot \vec{v}_2 + \right. \\ \left. 32 \hat{n} \times \vec{S}_1 \cdot \vec{v}_2 \hat{n} \cdot \vec{v}_1 \vec{v}_1 \cdot \vec{v}_1 \hat{n} \cdot \vec{v}_2 - 8 \vec{S}_1 \times \vec{v}_1 \cdot \vec{v}_2 \vec{v}_1 \cdot \vec{v}_2 \hat{n} \cdot \vec{v}_2 - 32 \hat{n} \times \vec{S}_1 \cdot \vec{v}_1 \hat{n} \cdot \vec{v}_1 \vec{v}_1 \cdot \vec{v}_2 \hat{n} \cdot \vec{v}_2 + \right. \\ \left. 48 \hat{n} \times \vec{S}_1 \cdot \vec{v}_2 \hat{n} \cdot \vec{v}_1 \vec{v}_1 \cdot \vec{v}_2 \hat{n} \cdot \vec{v}_2 - 48 \hat{n} \times \vec{S}_1 \cdot \vec{v}_1 \hat{n} \cdot \vec{v}_1 \vec{v}_2 \cdot \vec{v}_2 \hat{n} \cdot \vec{v}_2 + 10 \hat{n} \times \vec{S}_1 \cdot \vec{v}_1 (\vec{v}_1 \cdot \vec{v}_2)^2 - \right. \\ \left. 12 \hat{n} \times \vec{S}_1 \cdot \vec{v}_2 (\vec{v}_1 \cdot \vec{v}_2)^2 + 10 \vec{S}_1 \times \vec{v}_1 \cdot \vec{v}_2 \hat{n} \cdot \vec{v}_1 \vec{v}_1 \cdot \vec{v}_2 - 8 \hat{n} \times \vec{S}_1 \cdot \vec{v}_2 \vec{v}_1 \cdot \vec{v}_1 \vec{v}_1 \cdot \vec{v}_2 + 12 \vec{S}_1 \times \vec{v}_1 \cdot \vec{v}_2 \hat{n} \cdot \vec{v}_1 \vec{v}_2 \cdot \vec{v}_2 - \right. \\ \left. 2 \hat{n} \times \vec{S}_1 \cdot \vec{v}_1 \vec{v}_1 \cdot \vec{v}_1 \vec{v}_2 \cdot \vec{v}_2 + 8 \hat{n} \times \vec{S}_1 \cdot \vec{v}_2 \vec{v}_1 \cdot \vec{v}_1 \vec{v}_2 \cdot \vec{v}_2 + 4 \hat{n} \times \vec{S}_1 \cdot \vec{v}_1 \vec{v}_1 \cdot \vec{v}_2 \vec{v}_2 \cdot \vec{v}_2 \right) m_1 m_2 G^2 \}$$

$$\left\{ \text{DiagSet}[2, 2, 5], \right\}$$

$$\frac{1}{r^2} \left( 8 \vec{S}_1 \times \vec{v}_1 \cdot \vec{v}_2 \vec{a}_1 \cdot \vec{v}_2 + 2 \hat{n} \times \vec{S}_1 \cdot \vec{v}_2 \hat{n} \cdot \vec{v}_1 \vec{a}_1 \cdot \vec{v}_2 - 14 \hat{n} \times \vec{S}_1 \cdot \vec{v}_1 \hat{n} \cdot \vec{v}_2 \vec{a}_1 \cdot \vec{v}_2 + \right. \\ \left. 28 \hat{n} \times \vec{S}_1 \cdot \vec{v}_2 \hat{n} \cdot \vec{v}_2 \vec{v}_1 \cdot \vec{a}_1 + 4 \vec{S}_1 \times \vec{v}_1 \cdot \vec{v}_2 \vec{v}_1 \cdot \vec{a}_2 - 4 \hat{n} \times \vec{S}_1 \cdot \vec{v}_2 \hat{n} \cdot \vec{v}_1 \vec{v}_1 \cdot \vec{a}_2 - 8 \hat{n} \times \vec{S}_1 \cdot \vec{v}_1 \hat{n} \cdot \vec{v}_2 \vec{v}_1 \cdot \vec{a}_2 + \right. \\ \left. 8 \hat{n} \times \vec{S}_1 \cdot \vec{v}_2 \hat{n} \cdot \vec{a}_2 \vec{v}_1 \cdot \vec{v}_1 + 6 \hat{n} \times \vec{S}_1 \cdot \vec{v}_2 \hat{n} \cdot \vec{v}_2 \vec{v}_1 \cdot \vec{v}_1 + 8 \hat{n} \times \vec{S}_1 \cdot \vec{a}_2 \hat{n} \cdot \vec{v}_2 \vec{v}_1 \cdot \vec{v}_1 + 8 \vec{S}_1 \times \vec{a}_1 \cdot \vec{v}_2 \vec{v}_1 \cdot \vec{v}_2 + \right. \\ \left. 4 \vec{S}_1 \times \vec{v}_1 \cdot \vec{a}_2 \vec{v}_1 \cdot \vec{v}_2 + 2 \hat{n} \times \vec{S}_1 \cdot \vec{v}_2 \hat{n} \cdot \vec{a}_1 \vec{v}_1 \cdot \vec{v}_2 - 8 \hat{n} \times \vec{S}_1 \cdot \vec{v}_1 \hat{n} \cdot \vec{a}_2 \vec{v}_1 \cdot \vec{v}_2 - 6 \hat{n} \times \vec{S}_1 \cdot \vec{v}_2 \hat{n} \cdot \vec{v}_1 \vec{v}_1 \cdot \vec{v}_2 - \right. \\ \left. 4 \hat{n} \times \vec{S}_1 \cdot \vec{a}_2 \hat{n} \cdot \vec{v}_1 \vec{v}_1 \cdot \vec{v}_2 - 6 \hat{n} \times \vec{S}_1 \cdot \vec{v}_1 \hat{n} \cdot \vec{v}_2 \vec{v}_1 \cdot \vec{v}_2 - 14 \hat{n} \times \vec{S}_1 \cdot \vec{a}_1 \hat{n} \cdot \vec{v}_2 \vec{v}_1 \cdot \vec{v}_2 + 8 \hat{n} \times \vec{S}_1 \cdot \vec{v}_1 \hat{n} \cdot \vec{v}_1 \vec{v}_2 \cdot \vec{a}_2 - \right. \\ \left. 2 \hat{n} \times \vec{S}_1 \cdot \vec{v}_1 \hat{n} \cdot \vec{a}_1 \vec{v}_2 \cdot \vec{v}_2 + 6 \hat{n} \times \vec{S}_1 \cdot \vec{v}_1 \hat{n} \cdot \vec{v}_1 \vec{v}_2 \cdot \vec{v}_2 - 2 \hat{n} \times \vec{S}_1 \cdot \vec{a}_1 \hat{n} \cdot \vec{v}_1 \vec{v}_2 \cdot \vec{v}_2 \right) m_1 m_2 G^2 + \frac{1}{r^3} \\ \left( 16 \hat{n} \times \vec{S}_1 \cdot \vec{v}_2 \vec{v}_1 \cdot \vec{v}_2 (\hat{n} \cdot \vec{v}_1)^2 - 16 \hat{n} \times \vec{S}_1 \cdot \vec{v}_1 \vec{v}_2 \cdot \vec{v}_2 (\hat{n} \cdot \vec{v}_1)^2 - 32 \hat{n} \times \vec{S}_1 \cdot \vec{v}_2 \hat{n} \cdot \vec{v}_2 \vec{v}_1 \cdot \vec{v}_1 \hat{n} \cdot \vec{v}_1 - \right. \\ \left. 2 \vec{S}_1 \times \vec{v}_1 \cdot \vec{v}_2 \vec{v}_1 \cdot \vec{v}_2 \hat{n} \cdot \vec{v}_1 + 32 \hat{n} \times \vec{S}_1 \cdot \vec{v}_1 \hat{n} \cdot \vec{v}_2 \vec{v}_1 \cdot \vec{v}_2 \hat{n} \cdot \vec{v}_1 - 16 \hat{n} \times \vec{S}_1 \cdot \vec{v}_2 \hat{n} \cdot \vec{v}_2 \vec{v}_1 \cdot \vec{v}_2 \hat{n} \cdot \vec{v}_1 - \right. \\ \left. 4 \vec{S}_1 \times \vec{v}_1 \cdot \vec{v}_2 \vec{v}_2 \cdot \vec{v}_2 \hat{n} \cdot \vec{v}_1 + 16 \hat{n} \times \vec{S}_1 \cdot \vec{v}_1 \hat{n} \cdot \vec{v}_2 \vec{v}_2 \cdot \vec{v}_2 \hat{n} \cdot \vec{v}_1 - 7 \hat{n} \times \vec{S}_1 \cdot \vec{v}_1 (\vec{v}_1 \cdot \vec{v}_2)^2 + \right. \\ \left. 4 \hat{n} \times \vec{S}_1 \cdot \vec{v}_2 (\vec{v}_1 \cdot \vec{v}_2)^2 + 32 \hat{n} \times \vec{S}_1 \cdot \vec{v}_2 (\hat{n} \cdot \vec{v}_2)^2 \vec{v}_1 \cdot \vec{v}_1 - 10 \vec{S}_1 \times \vec{v}_1 \cdot \vec{v}_2 \hat{n} \cdot \vec{v}_2 \vec{v}_1 \cdot \vec{v}_1 - \right. \\ \left. 32 \hat{n} \times \vec{S}_1 \cdot \vec{v}_1 (\hat{n} \cdot \vec{v}_2)^2 \vec{v}_1 \cdot \vec{v}_2 + 16 \vec{S}_1 \times \vec{v}_1 \cdot \vec{v}_2 \hat{n} \cdot \vec{v}_2 \vec{v}_1 \cdot \vec{v}_2 + 4 \hat{n} \times \vec{S}_1 \cdot \vec{v}_2 \vec{v}_1 \cdot \vec{v}_1 \vec{v}_1 \cdot \vec{v}_2 + \right. \\ \left. 3 \hat{n} \times \vec{S}_1 \cdot \vec{v}_1 \vec{v}_1 \cdot \vec{v}_1 \vec{v}_2 \cdot \vec{v}_2 - 8 \hat{n} \times \vec{S}_1 \cdot \vec{v}_2 \vec{v}_1 \cdot \vec{v}_1 \vec{v}_2 \cdot \vec{v}_2 + 4 \hat{n} \times \vec{S}_1 \cdot \vec{v}_1 \vec{v}_1 \cdot \vec{v}_2 \vec{v}_2 \cdot \vec{v}_2 \right) m_1 m_2 G^2 \Big\}$$

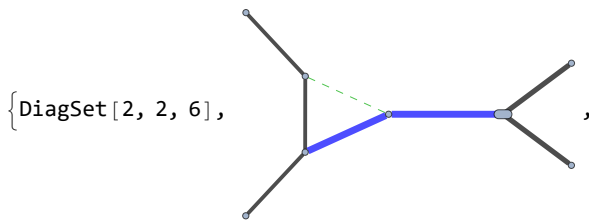

$$\frac{1}{r^2} G^2 m_2^2 \left( -16 \vec{a}_1 \cdot \vec{v}_2 \hat{n} \cdot \vec{v}_2 \hat{n} \times \vec{S}_1 \cdot \vec{v}_2 + 8 \vec{a}_2 \cdot \vec{v}_1 \hat{n} \cdot \vec{v}_2 \hat{n} \times \vec{S}_1 \cdot \vec{v}_2 - 16 \vec{a}_2 \cdot \vec{v}_2 \hat{n} \cdot \vec{v}_1 \hat{n} \times \vec{S}_1 \cdot \vec{v}_2 - \right. \\ \left. 16 \vec{a}_2 \cdot \vec{v}_2 \hat{n} \cdot \vec{v}_2 \hat{n} \times \vec{S}_1 \cdot \vec{v}_1 - 24 \vec{v}_1 \cdot \vec{v}_2 \hat{n} \cdot \vec{a}_2 \hat{n} \times \vec{S}_1 \cdot \vec{v}_2 - 8 \vec{v}_1 \cdot \vec{v}_2 \hat{n} \cdot \vec{v}_2 \hat{n} \times \vec{a}_2 \cdot \vec{S}_1 + 24 \vec{v}_2 \cdot \vec{v}_2 \hat{n} \cdot \vec{a}_2 \hat{n} \times \vec{S}_1 \cdot \vec{v}_1 - \right. \\ \left. 16 \vec{v}_2 \cdot \vec{v}_2 \hat{n} \cdot \vec{v}_1 \hat{n} \times \vec{a}_2 \cdot \vec{S}_1 - 16 \vec{v}_2 \cdot \vec{v}_2 \hat{n} \cdot \vec{v}_2 \hat{n} \times \vec{a}_1 \cdot \vec{S}_1 + 16 \vec{v}_1 \cdot \vec{v}_2 \vec{a}_2 \times \vec{S}_1 \cdot \vec{v}_2 + 8 \vec{v}_2 \cdot \vec{v}_2 \vec{a}_1 \times \vec{S}_1 \cdot \vec{v}_2 - \right. \\ \left. 4 \vec{v}_2 \cdot \vec{v}_2 \vec{a}_2 \times \vec{S}_1 \cdot \vec{v}_1 - 16 \vec{v}_1 \cdot \vec{v}_2 \hat{n} \cdot \vec{v}_2 \hat{n} \times \vec{S}_1 \cdot \vec{v}_2 + 16 \vec{v}_2 \cdot \vec{v}_2 \hat{n} \cdot \vec{v}_2 \hat{n} \times \vec{S}_1 \cdot \vec{v}_1 - 8 \vec{v}_2 \cdot \vec{v}_2 \vec{S}_1 \times \vec{v}_1 \cdot \vec{v}_2 \right) + \\ \frac{1}{r^3} G^2 m_2^2 \left( -16 (\vec{v}_1 \cdot \vec{v}_2)^2 \hat{n} \times \vec{S}_1 \cdot \vec{v}_2 + 16 \vec{v}_1 \cdot \vec{v}_2 \hat{n} \cdot \vec{v}_2 \vec{S}_1 \times \vec{v}_1 \cdot \vec{v}_2 + 64 \vec{v}_1 \cdot \vec{v}_2 \hat{n} \cdot \vec{v}_1 \hat{n} \cdot \vec{v}_2 \hat{n} \times \vec{S}_1 \cdot \vec{v}_2 + \right. \\ \left. 16 \vec{v}_2 \cdot \vec{v}_2 \vec{v}_1 \cdot \vec{v}_2 \hat{n} \times \vec{S}_1 \cdot \vec{v}_1 + 16 \vec{v}_2 \cdot \vec{v}_2 \hat{n} \cdot \vec{v}_1 \vec{S}_1 \times \vec{v}_1 \cdot \vec{v}_2 - 64 \vec{v}_2 \cdot \vec{v}_2 \hat{n} \cdot \vec{v}_1 \hat{n} \cdot \vec{v}_2 \hat{n} \times \vec{S}_1 \cdot \vec{v}_1 \right) \Big\}$$

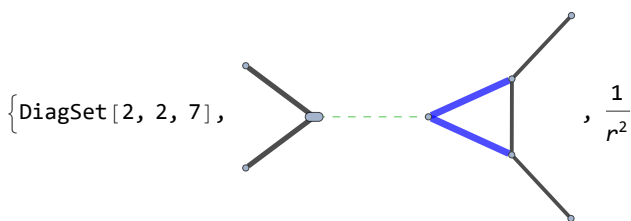

$$G^2 m_2^2 \left( 16 \vec{a}_2 \cdot \vec{v}_2 \hat{n} \cdot \vec{v}_2 \hat{n} \times \vec{S}_1 \cdot \vec{v}_2 + 16 \vec{v}_2 \cdot \vec{v}_2 \hat{n} \cdot \vec{v}_2 \hat{n} \times \vec{a}_2 \cdot \vec{S}_1 - 8 \vec{v}_2 \cdot \vec{v}_2 \vec{a}_2 \times \vec{S}_1 \cdot \vec{v}_2 \right) \Big\}$$

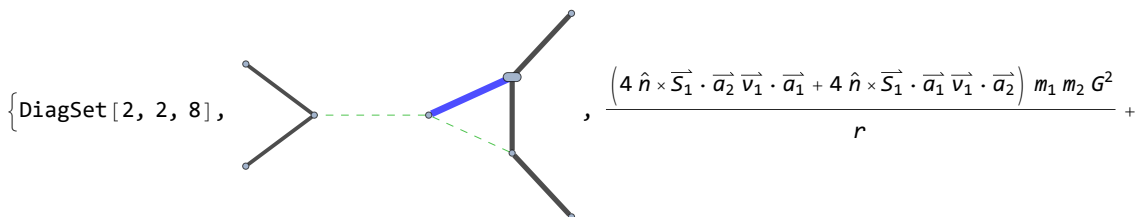

$$\frac{1}{r^2} \left( 4 \vec{S}_1 \times \vec{v}_1 \cdot \vec{v}_2 \vec{v}_1 \cdot \vec{a}_1 + 8 \hat{n} \times \vec{S}_1 \cdot \vec{v}_2 \hat{n} \cdot \vec{v}_2 \vec{v}_1 \cdot \vec{a}_1 - 2 \hat{n} \times \vec{S}_1 \cdot \vec{v}_1 \hat{n} \cdot \vec{v}_1 \vec{v}_1 \cdot \vec{a}_2 + 6 \vec{S}_1 \times \vec{v}_1 \cdot \vec{v}_2 \vec{v}_1 \cdot \vec{v}_1 + \right.$$

$$\begin{aligned}
& 8 \vec{S}_1 \times \vec{a}_1 \cdot \vec{v}_2 \vec{v}_1 \cdot \vec{v}_1 - 2 \vec{S}_1 \times \vec{v}_1 \cdot \vec{a}_2 \vec{v}_1 \cdot \vec{v}_1 - 2 \hat{n} \times \vec{S}_1 \cdot \vec{a}_2 \hat{n} \cdot \vec{v}_1 \vec{v}_1 \cdot \vec{v}_1 - 4 \vec{S}_1 \times \vec{a}_1 \cdot \vec{v}_2 \vec{v}_1 \cdot \vec{v}_2 - 8 \vec{S}_1 \times \vec{v}_1 \cdot \vec{a}_1 \vec{v}_1 \cdot \vec{v}_2 - \\
& 16 \hat{n} \times \vec{S}_1 \cdot \vec{v}_1 \hat{n} \cdot \vec{a}_1 \vec{v}_1 \cdot \vec{v}_2 - 24 \hat{n} \times \vec{S}_1 \cdot \vec{v}_1 \hat{n} \cdot \vec{v}_1 \vec{v}_1 \cdot \vec{v}_2 - 32 \hat{n} \times \vec{S}_1 \cdot \vec{a}_1 \hat{n} \cdot \vec{v}_1 \vec{v}_1 \cdot \vec{v}_2 + 8 \hat{n} \times \vec{S}_1 \cdot \vec{a}_1 \hat{n} \cdot \vec{v}_2 \vec{v}_1 \cdot \vec{v}_2 \Big) \\
& m_1 m_2 G^2 + \frac{1}{r^3} \Big( 16 \hat{n} \times \vec{S}_1 \cdot \vec{v}_1 \vec{v}_1 \cdot \vec{v}_2 (\hat{n} \cdot \vec{v}_1)^2 - 3 \vec{S}_1 \times \vec{v}_1 \cdot \vec{v}_2 \vec{v}_1 \cdot \vec{v}_1 \hat{n} \cdot \vec{v}_1 - 8 \hat{n} \times \vec{S}_1 \cdot \vec{v}_2 \hat{n} \cdot \vec{v}_2 \vec{v}_1 \cdot \vec{v}_1 \hat{n} \cdot \vec{v}_1 + \\
& 2 \vec{S}_1 \times \vec{v}_1 \cdot \vec{v}_2 \vec{v}_1 \cdot \vec{v}_2 \hat{n} \cdot \vec{v}_1 - 8 \hat{n} \times \vec{S}_1 \cdot \vec{v}_1 \hat{n} \cdot \vec{v}_2 \vec{v}_1 \cdot \vec{v}_2 \hat{n} \cdot \vec{v}_1 - \vec{S}_1 \times \vec{v}_1 \cdot \vec{v}_2 \vec{v}_2 \cdot \vec{v}_2 \hat{n} \cdot \vec{v}_1 - \\
& 3 \hat{n} \times \vec{S}_1 \cdot \vec{v}_2 (\vec{v}_1 \cdot \vec{v}_1)^2 + 2 \hat{n} \times \vec{S}_1 \cdot \vec{v}_1 (\vec{v}_1 \cdot \vec{v}_2)^2 - 4 \vec{S}_1 \times \vec{v}_1 \cdot \vec{v}_2 \hat{n} \cdot \vec{v}_2 \vec{v}_1 \cdot \vec{v}_1 - \hat{n} \times \vec{S}_1 \cdot \vec{v}_1 \vec{v}_1 \cdot \vec{v}_1 \vec{v}_1 \cdot \vec{v}_2 + \\
& 2 \hat{n} \times \vec{S}_1 \cdot \vec{v}_2 \vec{v}_1 \cdot \vec{v}_1 \vec{v}_1 \cdot \vec{v}_2 - 3 \hat{n} \times \vec{S}_1 \cdot \vec{v}_2 \vec{v}_1 \cdot \vec{v}_1 \vec{v}_2 \cdot \vec{v}_2 + 4 \hat{n} \times \vec{S}_1 \cdot \vec{v}_1 \vec{v}_1 \cdot \vec{v}_2 \vec{v}_2 \cdot \vec{v}_2 \Big) m_1 m_2 G^2 \Big\}
\end{aligned}$$

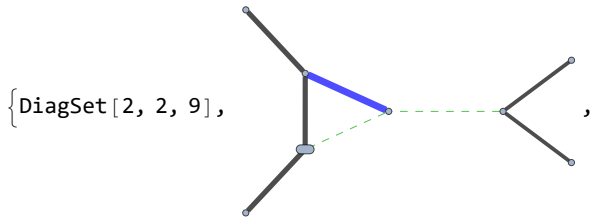

$$\begin{aligned}
& \frac{1}{r^2} G^2 m_1 m_2 \Big( -16 (\hat{n} \cdot \vec{v}_1)^2 \vec{S}_1 \times \vec{a}_1 \cdot \vec{v}_2 - 6 \vec{v}_1 \cdot \vec{a}_2 \hat{n} \cdot \vec{v}_1 \hat{n} \times \vec{S}_1 \cdot \vec{v}_1 - 8 \vec{v}_1 \cdot \vec{v}_2 \vec{S}_1 \times \vec{v}_1 \cdot \vec{a}_1 - \\
& 16 (\hat{n} \cdot \vec{v}_1)^2 \vec{S}_1 \times \vec{v}_1 \cdot \vec{v}_2 + 8 \vec{v}_1 \cdot \vec{v}_2 \hat{n} \cdot \vec{v}_2 \hat{n} \times \vec{S}_1 \cdot \vec{v}_1 - 4 \vec{v}_1 \cdot \vec{v}_2 \vec{S}_1 \times \vec{v}_1 \cdot \vec{v}_2 \Big) + \frac{4 G^2 m_1 m_2 \vec{v}_1 \cdot \vec{a}_2 \hat{n} \times \vec{S}_1 \cdot \vec{v}_1}{r} + \\
& \frac{1}{r^3} G^2 m_1 m_2 \Big( 12 (\hat{n} \cdot \vec{v}_1)^3 \vec{S}_1 \times \vec{v}_1 \cdot \vec{v}_2 + 12 \vec{v}_1 \cdot \vec{v}_1 (\hat{n} \cdot \vec{v}_1)^2 \hat{n} \times \vec{S}_1 \cdot \vec{v}_2 + 36 \vec{v}_1 \cdot \vec{v}_2 (\hat{n} \cdot \vec{v}_1)^2 \hat{n} \times \vec{S}_1 \cdot \vec{v}_1 + \\
& 12 \vec{v}_2 \cdot \vec{v}_2 (\hat{n} \cdot \vec{v}_1)^2 \hat{n} \times \vec{S}_1 \cdot \vec{v}_2 - 2 \vec{v}_1 \cdot \vec{v}_1 \hat{n} \cdot \vec{v}_1 \vec{S}_1 \times \vec{v}_1 \cdot \vec{v}_2 + 6 \vec{v}_1 \cdot \vec{v}_2 \hat{n} \cdot \vec{v}_1 \vec{S}_1 \times \vec{v}_1 \cdot \vec{v}_2 - \\
& 24 \vec{v}_1 \cdot \vec{v}_2 \hat{n} \cdot \vec{v}_2 \hat{n} \cdot \vec{v}_1 \hat{n} \times \vec{S}_1 \cdot \vec{v}_1 + 4 \vec{v}_2 \cdot \vec{v}_2 \hat{n} \cdot \vec{v}_1 \vec{S}_1 \times \vec{v}_1 \cdot \vec{v}_2 - 2 (\vec{v}_1 \cdot \vec{v}_1)^2 \hat{n} \times \vec{S}_1 \cdot \vec{v}_2 + \\
& 6 (\vec{v}_1 \cdot \vec{v}_2)^2 \hat{n} \times \vec{S}_1 \cdot \vec{v}_1 - 10 \vec{v}_1 \cdot \vec{v}_1 \vec{v}_1 \cdot \vec{v}_2 \hat{n} \times \vec{S}_1 \cdot \vec{v}_1 - 2 \vec{v}_1 \cdot \vec{v}_1 \vec{v}_2 \cdot \vec{v}_2 \hat{n} \times \vec{S}_1 \cdot \vec{v}_2 - \vec{v}_1 \cdot \vec{v}_2 \vec{v}_2 \cdot \vec{v}_2 \hat{n} \times \vec{S}_1 \cdot \vec{v}_1 \Big) \Big\}
\end{aligned}$$

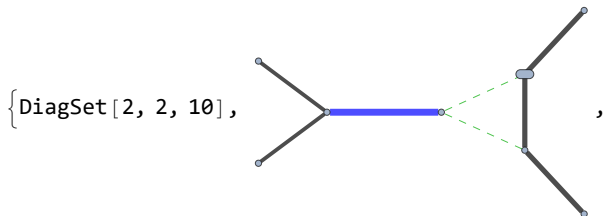

$$\begin{aligned}
& \frac{1}{r^2} G^2 m_1 m_2 \Big( -4 (\hat{n} \cdot \vec{v}_2)^2 \vec{S}_1 \times \vec{v}_1 \cdot \vec{a}_1 - 6 \vec{a}_1 \cdot \vec{v}_2 \hat{n} \cdot \vec{v}_1 \hat{n} \times \vec{S}_1 \cdot \vec{v}_2 - 2 \vec{a}_1 \cdot \vec{v}_2 \vec{S}_1 \times \vec{v}_1 \cdot \vec{v}_2 - \\
& 8 \vec{v}_1 \cdot \vec{v}_2 \vec{S}_1 \times \vec{a}_1 \cdot \vec{v}_2 - 4 \vec{v}_2 \cdot \vec{v}_2 \vec{S}_1 \times \vec{v}_1 \cdot \vec{a}_1 - 2 \vec{v}_1 \cdot \vec{v}_2 \hat{n} \cdot \vec{v}_1 \hat{n} \times \vec{S}_1 \cdot \vec{v}_2 - 10 \vec{v}_1 \cdot \vec{v}_2 \vec{S}_1 \times \vec{v}_1 \cdot \vec{v}_2 \Big) + \\
& \frac{4 G^2 m_1 m_2 \vec{a}_1 \cdot \vec{v}_2 \hat{n} \times \vec{S}_1 \cdot \vec{v}_2}{r} + \frac{1}{r^3} G^2 m_1 m_2 \Big( 4 \vec{v}_1 \cdot \vec{v}_2 (\hat{n} \cdot \vec{v}_1)^2 \hat{n} \times \vec{S}_1 \cdot \vec{v}_2 + 3 \vec{v}_1 \cdot \vec{v}_2 \hat{n} \cdot \vec{v}_1 \vec{S}_1 \times \vec{v}_1 \cdot \vec{v}_2 + \\
& 7 (\vec{v}_1 \cdot \vec{v}_2)^2 \hat{n} \times \vec{S}_1 \cdot \vec{v}_1 - 8 \vec{v}_1 \cdot \vec{v}_1 (\hat{n} \cdot \vec{v}_2)^2 \hat{n} \times \vec{S}_1 \cdot \vec{v}_1 + 4 \vec{v}_1 \cdot \vec{v}_1 \hat{n} \cdot \vec{v}_2 \vec{S}_1 \times \vec{v}_1 \cdot \vec{v}_2 - \vec{v}_1 \cdot \vec{v}_1 \vec{v}_1 \cdot \vec{v}_2 \hat{n} \times \vec{S}_1 \cdot \vec{v}_2 - \\
& 2 \vec{v}_2 \cdot \vec{v}_2 (\hat{n} \cdot \vec{v}_2)^2 \hat{n} \times \vec{S}_1 \cdot \vec{v}_1 - 4 \vec{v}_1 \cdot \vec{v}_1 \vec{v}_2 \cdot \vec{v}_2 \hat{n} \times \vec{S}_1 \cdot \vec{v}_1 + \vec{v}_1 \cdot \vec{v}_2 \vec{v}_2 \cdot \vec{v}_2 \hat{n} \times \vec{S}_1 \cdot \vec{v}_2 \Big) \Big\}
\end{aligned}$$

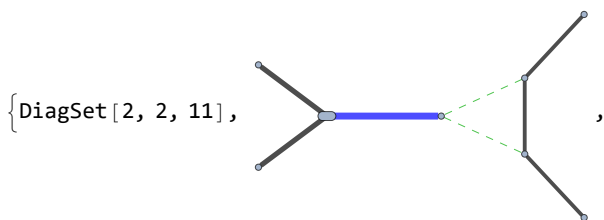

$$\frac{1}{r^2} G^2 m_2^2 \left( 8 \vec{a}_2 \cdot \vec{v}_1 \hat{n} \cdot \vec{v}_2 \hat{n} \times \vec{S}_1 \cdot \vec{v}_2 - 8 \vec{v}_1 \cdot \vec{v}_2 \hat{n} \cdot \vec{v}_2 \hat{n} \times \vec{a}_2 \cdot \vec{S}_1 + 2 \vec{v}_2 \cdot \vec{v}_2 \hat{n} \cdot \vec{a}_1 \hat{n} \times \vec{S}_1 \cdot \vec{v}_1 - \right. \\ \left. 4 \vec{v}_2 \cdot \vec{v}_2 \hat{n} \cdot \vec{v}_1 \hat{n} \times \vec{a}_1 \cdot \vec{S}_1 - 4 \vec{a}_1 \cdot \vec{v}_2 \vec{S}_1 \times \vec{v}_1 \cdot \vec{v}_2 + 8 \vec{v}_1 \cdot \vec{v}_2 \vec{a}_1 \times \vec{S}_1 \cdot \vec{v}_2 + 4 \vec{v}_1 \cdot \vec{v}_2 \vec{a}_2 \times \vec{S}_1 \cdot \vec{v}_2 - \right. \\ \left. 2 \vec{v}_2 \cdot \vec{v}_2 \vec{a}_1 \times \vec{S}_1 \cdot \vec{v}_1 + 3 \vec{v}_2 \cdot \vec{v}_2 \hat{n} \cdot \vec{v}_1 \hat{n} \times \vec{S}_1 \cdot \vec{v}_1 - 6 \vec{v}_1 \cdot \vec{v}_2 \vec{S}_1 \times \vec{v}_1 \cdot \vec{v}_2 \right) - \frac{8 G^2 m_2^2 \vec{a}_2 \cdot \vec{v}_1 \hat{n} \times \vec{a}_2 \cdot \vec{S}_1}{r} + \\ \frac{1}{r^3} G^2 m_2^2 \left( -8 \vec{v}_2 \cdot \vec{v}_2 (\hat{n} \cdot \vec{v}_1)^2 \hat{n} \times \vec{S}_1 \cdot \vec{v}_1 + 4 \vec{v}_1 \cdot \vec{v}_2 \hat{n} \cdot \vec{v}_1 \vec{S}_1 \times \vec{v}_1 \cdot \vec{v}_2 + 4 (\vec{v}_1 \cdot \vec{v}_2)^2 \hat{n} \times \vec{S}_1 \cdot \vec{v}_1 - \right. \\ \left. 6 (\vec{v}_2 \cdot \vec{v}_2)^2 \hat{n} \times \vec{S}_1 \cdot \vec{v}_1 + 8 \vec{v}_1 \cdot \vec{v}_2 (\hat{n} \cdot \vec{v}_2)^2 \hat{n} \times \vec{S}_1 \cdot \vec{v}_2 - \vec{v}_1 \cdot \vec{v}_1 \vec{v}_2 \cdot \vec{v}_2 \hat{n} \times \vec{S}_1 \cdot \vec{v}_1 + 4 \vec{v}_1 \cdot \vec{v}_2 \vec{v}_2 \cdot \vec{v}_2 \hat{n} \times \vec{S}_1 \cdot \vec{v}_2 \right) \Big\}$$

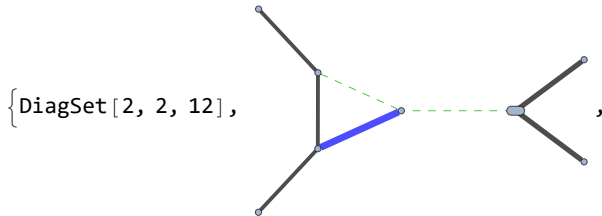

$$\frac{1}{r^2} G^2 m_2^2 \left( 16 (\hat{n} \cdot \vec{v}_2)^2 \vec{a}_1 \times \vec{S}_1 \cdot \vec{v}_2 - 16 \vec{a}_2 \cdot \vec{v}_2 \hat{n} \cdot \vec{v}_1 \hat{n} \times \vec{S}_1 \cdot \vec{v}_2 - 8 \vec{a}_2 \cdot \vec{v}_2 \vec{S}_1 \times \vec{v}_1 \cdot \vec{v}_2 - 8 \vec{v}_2 \cdot \vec{v}_2 \vec{a}_1 \times \vec{S}_1 \cdot \vec{v}_2 - \right. \\ \left. 16 (\hat{n} \cdot \vec{v}_2)^2 \vec{S}_1 \times \vec{v}_1 \cdot \vec{v}_2 + 8 \vec{v}_2 \cdot \vec{v}_2 \hat{n} \cdot \vec{v}_2 \hat{n} \times \vec{S}_1 \cdot \vec{v}_2 + 8 \vec{v}_2 \cdot \vec{v}_2 \vec{S}_1 \times \vec{v}_1 \cdot \vec{v}_2 \right) + \frac{8 G^2 m_2^2 \vec{a}_2 \cdot \vec{v}_2 \hat{n} \times \vec{S}_1 \cdot \vec{v}_2}{r} + \\ \frac{1}{r^3} G^2 m_2^2 \left( 16 \hat{n} \cdot \vec{v}_1 (\hat{n} \cdot \vec{v}_2)^2 \vec{S}_1 \times \vec{v}_1 \cdot \vec{v}_2 + 48 \vec{v}_1 \cdot \vec{v}_2 (\hat{n} \cdot \vec{v}_2)^2 \hat{n} \times \vec{S}_1 \cdot \vec{v}_1 + 32 \vec{v}_2 \cdot \vec{v}_2 (\hat{n} \cdot \vec{v}_2)^2 \hat{n} \times \vec{S}_1 \cdot \vec{v}_2 - \right. \\ \left. 32 \vec{v}_1 \cdot \vec{v}_2 \hat{n} \cdot \vec{v}_2 \vec{S}_1 \times \vec{v}_1 \cdot \vec{v}_2 - 8 \vec{v}_2 \cdot \vec{v}_2 \hat{n} \cdot \vec{v}_2 \vec{S}_1 \times \vec{v}_1 \cdot \vec{v}_2 - 32 \vec{v}_2 \cdot \vec{v}_2 \hat{n} \cdot \vec{v}_1 \hat{n} \cdot \vec{v}_2 \hat{n} \times \vec{S}_1 \cdot \vec{v}_2 - \right. \\ \left. 8 (\vec{v}_2 \cdot \vec{v}_2)^2 \hat{n} \times \vec{S}_1 \cdot \vec{v}_2 - 4 \vec{v}_2 \cdot \vec{v}_2 \hat{n} \cdot \vec{v}_1 \vec{S}_1 \times \vec{v}_1 \cdot \vec{v}_2 - 12 \vec{v}_1 \cdot \vec{v}_2 \vec{v}_2 \cdot \vec{v}_2 \hat{n} \times \vec{S}_1 \cdot \vec{v}_1 + 8 \vec{v}_1 \cdot \vec{v}_2 \vec{v}_2 \cdot \vec{v}_2 \hat{n} \times \vec{S}_1 \cdot \vec{v}_2 \right) \Big\}$$

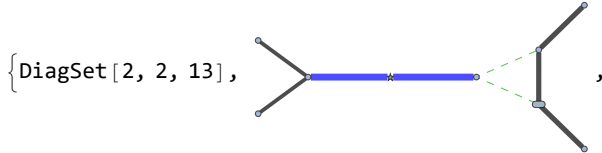

$$\frac{1}{r} \left( -\frac{2}{3} \vec{S}_1 \times \vec{v}_1 \cdot \vec{v}_2 \hat{n} \cdot \vec{a}_2 - \frac{2}{3} \vec{S}_1 \times \vec{a}_1 \cdot \vec{v}_2 \hat{n} \cdot \vec{a}_2 - \frac{2}{3} \hat{n} \times \vec{S}_1 \cdot \vec{v}_1 \hat{n} \cdot \vec{v}_2 \hat{n} \cdot \vec{a}_2 - \frac{2}{3} \hat{n} \times \vec{S}_1 \cdot \vec{a}_1 \hat{n} \cdot \vec{v}_2 \hat{n} \cdot \vec{a}_2 - \right. \\ \left. \frac{2}{3} \vec{S}_1 \times \vec{v}_1 \cdot \vec{a}_2 \hat{n} \cdot \vec{v}_2 - \frac{2}{3} \vec{S}_1 \times \vec{a}_1 \cdot \vec{a}_2 \hat{n} \cdot \vec{v}_2 + \hat{n} \times \vec{S}_1 \cdot \vec{v}_2 \vec{a}_1 \cdot \vec{a}_2 + \hat{n} \times \vec{S}_1 \cdot \vec{a}_2 \vec{a}_1 \cdot \vec{v}_2 + \right. \\ \left. \hat{n} \times \vec{S}_1 \cdot \vec{v}_2 \vec{v}_1 \cdot \vec{a}_2 + \hat{n} \times \vec{S}_1 \cdot \vec{a}_2 \vec{v}_1 \cdot \vec{v}_2 - \frac{2}{3} \hat{n} \times \vec{S}_1 \cdot \vec{v}_1 \vec{v}_2 \cdot \vec{a}_2 - \frac{2}{3} \hat{n} \times \vec{S}_1 \cdot \vec{a}_1 \vec{v}_2 \cdot \vec{a}_2 \right) m_1 m_2 G^2 + \\ \frac{1}{r^2} \left( -\frac{4}{3} \hat{n} \times \vec{S}_1 \cdot \vec{v}_1 (\hat{n} \cdot \vec{v}_2)^3 - \frac{4}{3} \hat{n} \times \vec{S}_1 \cdot \vec{a}_1 (\hat{n} \cdot \vec{v}_2)^3 - \frac{1}{3} \vec{S}_1 \times \vec{v}_1 \cdot \vec{v}_2 (\hat{n} \cdot \vec{v}_2)^2 - \vec{S}_1 \times \vec{a}_1 \cdot \vec{v}_2 (\hat{n} \cdot \vec{v}_2)^2 + \right. \\ \left. \frac{4}{3} \vec{S}_1 \times \vec{v}_1 \cdot \vec{a}_2 \hat{n} \cdot \vec{v}_1 \hat{n} \cdot \vec{v}_2 + \frac{8}{3} \hat{n} \times \vec{S}_1 \cdot \vec{v}_1 \hat{n} \cdot \vec{a}_2 \hat{n} \cdot \vec{v}_1 \hat{n} \cdot \vec{v}_2 + 2 \hat{n} \times \vec{S}_1 \cdot \vec{v}_2 \vec{a}_1 \cdot \vec{v}_2 \hat{n} \cdot \vec{v}_2 - \right. \\ \left. \frac{2}{3} \hat{n} \times \vec{S}_1 \cdot \vec{v}_1 \vec{v}_1 \cdot \vec{a}_2 \hat{n} \cdot \vec{v}_2 + 2 \hat{n} \times \vec{S}_1 \cdot \vec{v}_2 \vec{v}_1 \cdot \vec{v}_2 \hat{n} \cdot \vec{v}_2 + \frac{4}{3} \vec{S}_1 \times \vec{v}_1 \cdot \vec{v}_2 \hat{n} \cdot \vec{a}_2 \hat{n} \cdot \vec{v}_1 - \right. \\ \left. \frac{5}{3} \vec{S}_1 \times \vec{v}_1 \cdot \vec{v}_2 \vec{v}_1 \cdot \vec{a}_2 - 2 \hat{n} \times \vec{S}_1 \cdot \vec{v}_2 \hat{n} \cdot \vec{v}_1 \vec{v}_1 \cdot \vec{a}_2 - \frac{5}{3} \vec{S}_1 \times \vec{v}_1 \cdot \vec{a}_2 \vec{v}_1 \cdot \vec{v}_2 - \frac{2}{3} \hat{n} \times \vec{S}_1 \cdot \vec{v}_1 \hat{n} \cdot \vec{a}_2 \vec{v}_1 \cdot \vec{v}_2 - \right. \\ \left. 2 \hat{n} \times \vec{S}_1 \cdot \vec{a}_2 \hat{n} \cdot \vec{v}_1 \vec{v}_1 \cdot \vec{v}_2 + \frac{4}{3} \hat{n} \times \vec{S}_1 \cdot \vec{v}_1 \hat{n} \cdot \vec{v}_1 \vec{v}_2 \cdot \vec{a}_2 + \vec{S}_1 \times \vec{v}_1 \cdot \vec{v}_2 \vec{v}_2 \cdot \vec{v}_2 + \vec{S}_1 \times \vec{a}_1 \cdot \vec{v}_2 \vec{v}_2 \cdot \vec{v}_2 \right) m_1 m_2 G^2 + \frac{1}{r^3} \\ \left( 8 \hat{n} \times \vec{S}_1 \cdot \vec{v}_1 \hat{n} \cdot \vec{v}_1 (\hat{n} \cdot \vec{v}_2)^3 + 4 \vec{S}_1 \times \vec{v}_1 \cdot \vec{v}_2 \hat{n} \cdot \vec{v}_1 (\hat{n} \cdot \vec{v}_2)^2 - 4 \hat{n} \times \vec{S}_1 \cdot \vec{v}_1 \vec{v}_1 \cdot \vec{v}_2 (\hat{n} \cdot \vec{v}_2)^2 - 4 \vec{S}_1 \times \vec{v}_1 \cdot \vec{v}_2 \vec{v}_1 \cdot \vec{v}_2 \hat{n} \cdot \vec{v}_2 - \right. \\ \left. 8 \hat{n} \times \vec{S}_1 \cdot \vec{v}_2 \hat{n} \cdot \vec{v}_1 \vec{v}_1 \cdot \vec{v}_2 \hat{n} \cdot \vec{v}_2 + 2 \hat{n} \times \vec{S}_1 \cdot \vec{v}_2 (\vec{v}_1 \cdot \vec{v}_2)^2 - 2 \vec{S}_1 \times \vec{v}_1 \cdot \vec{v}_2 \hat{n} \cdot \vec{v}_1 \vec{v}_2 \cdot \vec{v}_2 \right) m_1 m_2 G^2 \Big\}$$

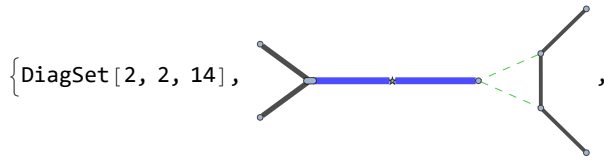

$$\begin{aligned} & \frac{1}{r^2} G^2 m_2^2 \left( 8 \vec{a}_1 \cdot \vec{v}_2 \hat{n} \cdot \vec{v}_2 \hat{n} \times \vec{S}_1 \cdot \vec{v}_2 - 8 \vec{a}_2 \cdot \vec{v}_1 \hat{n} \cdot \vec{v}_1 \hat{n} \times \vec{S}_1 \cdot \vec{v}_2 + 12 \vec{a}_2 \cdot \vec{v}_2 \hat{n} \cdot \vec{v}_1 \hat{n} \times \vec{S}_1 \cdot \vec{v}_1 + \right. \\ & 8 \vec{v}_1 \cdot \vec{v}_2 \hat{n} \cdot \vec{v}_1 \hat{n} \times \vec{a}_2 \cdot \vec{S}_1 + 6 \vec{v}_2 \cdot \vec{v}_2 \hat{n} \cdot \vec{v}_2 \hat{n} \times \vec{a}_1 \cdot \vec{S}_1 - 4 \vec{a}_2 \cdot \vec{v}_1 \vec{S}_1 \times \vec{v}_1 \cdot \vec{v}_2 - 4 \vec{v}_1 \cdot \vec{v}_2 \vec{a}_2 \times \vec{S}_1 \cdot \vec{v}_1 - \\ & \left. 3 \vec{v}_2 \cdot \vec{v}_2 \vec{a}_1 \times \vec{S}_1 \cdot \vec{v}_2 + 8 \vec{v}_1 \cdot \vec{v}_2 \hat{n} \cdot \vec{v}_2 \hat{n} \times \vec{S}_1 \cdot \vec{v}_2 - 6 \vec{v}_2 \cdot \vec{v}_2 \hat{n} \cdot \vec{v}_2 \hat{n} \times \vec{S}_1 \cdot \vec{v}_1 + 3 \vec{v}_2 \cdot \vec{v}_2 \vec{S}_1 \times \vec{v}_1 \cdot \vec{v}_2 \right) + \\ & \frac{1}{r} G^2 m_2^2 \left( 4 \vec{a}_1 \cdot \vec{a}_2 \hat{n} \times \vec{S}_1 \cdot \vec{v}_2 - 4 \vec{a}_1 \cdot \vec{v}_2 \hat{n} \times \vec{a}_2 \cdot \vec{S}_1 + 4 \vec{a}_2 \cdot \vec{v}_1 \hat{n} \times \vec{S}_1 \cdot \vec{v}_2 - 6 \vec{a}_2 \cdot \vec{v}_2 \hat{n} \times \vec{S}_1 \cdot \vec{v}_1 + \right. \\ & \left. 6 \vec{a}_2 \cdot \vec{v}_2 \hat{n} \times \vec{a}_1 \cdot \vec{S}_1 - 4 \vec{v}_1 \cdot \vec{v}_2 \hat{n} \times \vec{a}_2 \cdot \vec{S}_1 \right) + \frac{1}{r^3} \\ & G^2 m_2^2 \left( 8 (\vec{v}_1 \cdot \vec{v}_2)^2 \hat{n} \times \vec{S}_1 \cdot \vec{v}_2 - 8 \vec{v}_1 \cdot \vec{v}_2 \hat{n} \cdot \vec{v}_2 \vec{S}_1 \times \vec{v}_1 \cdot \vec{v}_2 - 32 \vec{v}_1 \cdot \vec{v}_2 \hat{n} \cdot \vec{v}_1 \hat{n} \cdot \vec{v}_2 \hat{n} \times \vec{S}_1 \cdot \vec{v}_2 - \right. \\ & \left. 6 \vec{v}_2 \cdot \vec{v}_2 \vec{v}_1 \cdot \vec{v}_2 \hat{n} \times \vec{S}_1 \cdot \vec{v}_1 - 6 \vec{v}_2 \cdot \vec{v}_2 \hat{n} \cdot \vec{v}_1 \vec{S}_1 \times \vec{v}_1 \cdot \vec{v}_2 + 24 \vec{v}_2 \cdot \vec{v}_2 \hat{n} \cdot \vec{v}_1 \hat{n} \cdot \vec{v}_2 \hat{n} \times \vec{S}_1 \cdot \vec{v}_1 \right) \} \end{aligned}$$

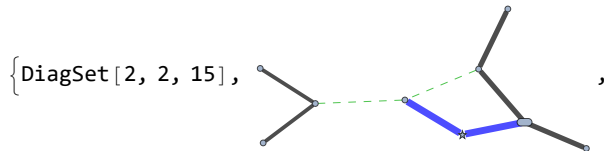

$$\begin{aligned} & \frac{1}{r} \left( 6 \vec{S}_1 \times \vec{v}_1 \cdot \vec{v}_2 \hat{n} \cdot \vec{a}_1 + 2 \vec{S}_1 \times \vec{a}_1 \cdot \vec{v}_2 \hat{n} \cdot \vec{a}_1 - 4 \vec{S}_1 \times \vec{v}_1 \cdot \vec{a}_2 \hat{n} \cdot \vec{a}_1 + 6 \vec{S}_1 \times \vec{v}_1 \cdot \vec{a}_1 \hat{n} \cdot \vec{a}_2 - \right. \\ & 4 \vec{S}_1 \times \vec{a}_1 \cdot \vec{v}_2 \hat{n} \cdot \vec{v}_1 + 2 \vec{S}_1 \times \vec{v}_1 \cdot \vec{a}_2 \hat{n} \cdot \vec{v}_1 + 6 \vec{S}_1 \times \vec{a}_1 \cdot \vec{a}_2 \hat{n} \cdot \vec{v}_1 - 6 \vec{S}_1 \times \vec{v}_1 \cdot \vec{a}_1 \hat{n} \cdot \vec{v}_2 + 2 \hat{n} \times \vec{S}_1 \cdot \vec{v}_2 \vec{a}_1 \cdot \vec{a}_1 - \\ & 2 \hat{n} \times \vec{S}_1 \cdot \vec{v}_1 \vec{a}_1 \cdot \vec{a}_2 - 2 \hat{n} \times \vec{S}_1 \cdot \vec{v}_1 \vec{a}_1 \cdot \vec{v}_2 - 4 \hat{n} \times \vec{S}_1 \cdot \vec{a}_1 \vec{a}_1 \cdot \vec{v}_2 + 2 \hat{n} \times \vec{S}_1 \cdot \vec{v}_2 \vec{v}_1 \cdot \vec{a}_1 + 2 \hat{n} \times \vec{S}_1 \cdot \vec{a}_2 \vec{v}_1 \cdot \vec{a}_1 - \\ & \left. 4 \hat{n} \times \vec{S}_1 \cdot \vec{v}_1 \vec{v}_1 \cdot \vec{a}_2 - 2 \hat{n} \times \vec{S}_1 \cdot \vec{a}_1 \vec{v}_1 \cdot \vec{a}_2 + 2 \hat{n} \times \vec{S}_1 \cdot \vec{a}_2 \vec{v}_1 \cdot \vec{v}_1 - 2 \hat{n} \times \vec{S}_1 \cdot \vec{a}_1 \vec{v}_1 \cdot \vec{v}_2 \right) m_1 m_2 G^2 + \\ & \frac{1}{r^3} \left( 2 \vec{S}_1 \times \vec{v}_1 \cdot \vec{v}_2 (\hat{n} \cdot \vec{v}_1)^3 - 4 \vec{S}_1 \times \vec{v}_1 \cdot \vec{v}_2 \hat{n} \cdot \vec{v}_2 (\hat{n} \cdot \vec{v}_1)^2 + 2 \hat{n} \times \vec{S}_1 \cdot \vec{v}_2 \vec{v}_1 \cdot \vec{v}_1 (\hat{n} \cdot \vec{v}_1)^2 + \right. \\ & 12 \hat{n} \times \vec{S}_1 \cdot \vec{v}_1 \vec{v}_1 \cdot \vec{v}_2 (\hat{n} \cdot \vec{v}_1)^2 - 2 \vec{S}_1 \times \vec{v}_1 \cdot \vec{v}_2 \vec{v}_1 \cdot \vec{v}_1 \hat{n} \cdot \vec{v}_1 - 8 \hat{n} \times \vec{S}_1 \cdot \vec{v}_2 \hat{n} \cdot \vec{v}_2 \vec{v}_1 \cdot \vec{v}_1 \hat{n} \cdot \vec{v}_1 + \\ & 6 \vec{S}_1 \times \vec{v}_1 \cdot \vec{v}_2 \vec{v}_1 \cdot \vec{v}_2 \hat{n} \cdot \vec{v}_1 - 16 \hat{n} \times \vec{S}_1 \cdot \vec{v}_1 \hat{n} \cdot \vec{v}_2 \vec{v}_1 \cdot \vec{v}_2 \hat{n} \cdot \vec{v}_1 - 2 \hat{n} \times \vec{S}_1 \cdot \vec{v}_2 (\vec{v}_1 \cdot \vec{v}_1)^2 + \\ & 4 \hat{n} \times \vec{S}_1 \cdot \vec{v}_1 (\vec{v}_1 \cdot \vec{v}_2)^2 + 2 \vec{S}_1 \times \vec{v}_1 \cdot \vec{v}_2 \hat{n} \cdot \vec{v}_2 \vec{v}_1 \cdot \vec{v}_1 + 2 \hat{n} \times \vec{S}_1 \cdot \vec{v}_2 \vec{v}_1 \cdot \vec{v}_1 \vec{v}_1 \cdot \vec{v}_2 \Big) m_1 m_2 G^2 + \frac{1}{r^2} \\ & \left( -3 \vec{S}_1 \times \vec{v}_1 \cdot \vec{v}_2 (\hat{n} \cdot \vec{v}_1)^2 - 7 \vec{S}_1 \times \vec{a}_1 \cdot \vec{v}_2 (\hat{n} \cdot \vec{v}_1)^2 - \vec{S}_1 \times \vec{v}_1 \cdot \vec{a}_2 (\hat{n} \cdot \vec{v}_1)^2 + 3 \vec{S}_1 \times \vec{v}_1 \cdot \vec{v}_2 \hat{n} \cdot \vec{a}_1 \hat{n} \cdot \vec{v}_1 + \right. \\ & 4 \vec{S}_1 \times \vec{v}_1 \cdot \vec{v}_2 \hat{n} \cdot \vec{v}_2 \hat{n} \cdot \vec{v}_1 + 12 \vec{S}_1 \times \vec{a}_1 \cdot \vec{v}_2 \hat{n} \cdot \vec{v}_2 \hat{n} \cdot \vec{v}_1 - 6 \vec{S}_1 \times \vec{v}_1 \cdot \vec{a}_1 \hat{n} \cdot \vec{v}_2 \hat{n} \cdot \vec{v}_1 - \hat{n} \times \vec{S}_1 \cdot \vec{v}_1 \vec{a}_1 \cdot \vec{v}_2 \hat{n} \cdot \vec{v}_1 - \\ & 6 \hat{n} \times \vec{S}_1 \cdot \vec{v}_2 \vec{v}_1 \cdot \vec{a}_1 \hat{n} \cdot \vec{v}_1 - 4 \hat{n} \times \vec{S}_1 \cdot \vec{v}_1 \vec{v}_1 \cdot \vec{a}_2 \hat{n} \cdot \vec{v}_1 - 2 \hat{n} \times \vec{S}_1 \cdot \vec{v}_2 \vec{v}_1 \cdot \vec{v}_1 \hat{n} \cdot \vec{v}_1 - 2 \hat{n} \times \vec{S}_1 \cdot \vec{a}_2 \vec{v}_1 \cdot \vec{v}_1 \hat{n} \cdot \vec{v}_1 + \\ & 12 \hat{n} \times \vec{S}_1 \cdot \vec{v}_1 \vec{v}_1 \cdot \vec{v}_2 \hat{n} \cdot \vec{v}_1 + 4 \hat{n} \times \vec{S}_1 \cdot \vec{a}_1 \vec{v}_1 \cdot \vec{v}_2 \hat{n} \cdot \vec{v}_1 + 12 \vec{S}_1 \times \vec{v}_1 \cdot \vec{a}_1 (\hat{n} \cdot \vec{v}_2)^2 - 8 \vec{S}_1 \times \vec{v}_1 \cdot \vec{v}_2 \hat{n} \cdot \vec{a}_1 \hat{n} \cdot \vec{v}_2 + \\ & 6 \vec{S}_1 \times \vec{v}_1 \cdot \vec{v}_2 \vec{a}_1 \cdot \vec{v}_2 - 4 \hat{n} \times \vec{S}_1 \cdot \vec{v}_1 \hat{n} \cdot \vec{v}_2 \vec{a}_1 \cdot \vec{v}_2 - 6 \vec{S}_1 \times \vec{v}_1 \cdot \vec{v}_2 \vec{v}_1 \cdot \vec{a}_1 + 3 \hat{n} \times \vec{S}_1 \cdot \vec{v}_1 \hat{n} \cdot \vec{v}_2 \vec{v}_1 \cdot \vec{a}_1 + \\ & 4 \hat{n} \times \vec{S}_1 \cdot \vec{v}_2 \hat{n} \cdot \vec{v}_2 \vec{v}_1 \cdot \vec{a}_1 - \vec{S}_1 \times \vec{v}_1 \cdot \vec{v}_2 \vec{v}_1 \cdot \vec{v}_1 + 6 \vec{S}_1 \times \vec{a}_1 \cdot \vec{v}_2 \vec{v}_1 \cdot \vec{v}_1 + \vec{S}_1 \times \vec{v}_1 \cdot \vec{a}_2 \vec{v}_1 \cdot \vec{v}_1 + 2 \hat{n} \times \vec{S}_1 \cdot \vec{v}_2 \hat{n} \cdot \vec{a}_1 \vec{v}_1 \cdot \vec{v}_1 + \\ & 4 \hat{n} \times \vec{S}_1 \cdot \vec{v}_2 \hat{n} \cdot \vec{v}_2 \vec{v}_1 \cdot \vec{v}_1 - 3 \hat{n} \times \vec{S}_1 \cdot \vec{a}_1 \hat{n} \cdot \vec{v}_2 \vec{v}_1 \cdot \vec{v}_1 + 2 \vec{S}_1 \times \vec{v}_1 \cdot \vec{v}_2 \vec{v}_1 \cdot \vec{v}_2 - 4 \vec{S}_1 \times \vec{a}_1 \cdot \vec{v}_2 \vec{v}_1 \cdot \vec{v}_2 + 7 \vec{S}_1 \times \vec{v}_1 \cdot \vec{a}_1 \vec{v}_1 \cdot \vec{v}_2 + \\ & \left. 5 \hat{n} \times \vec{S}_1 \cdot \vec{v}_1 \hat{n} \cdot \vec{a}_1 \vec{v}_1 \cdot \vec{v}_2 - 8 \hat{n} \times \vec{S}_1 \cdot \vec{v}_1 \hat{n} \cdot \vec{v}_2 \vec{v}_1 \cdot \vec{v}_2 - 4 \hat{n} \times \vec{S}_1 \cdot \vec{a}_1 \hat{n} \cdot \vec{v}_2 \vec{v}_1 \cdot \vec{v}_2 - 6 \vec{S}_1 \times \vec{v}_1 \cdot \vec{a}_1 \vec{v}_2 \cdot \vec{v}_2 \right) m_1 m_2 G^2 \} \end{aligned}$$



{DiagSet[2, 2, 16],

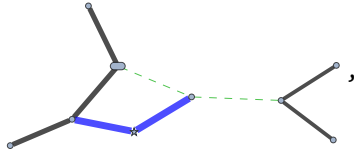

$$\frac{1}{r} \left( -8 \hat{n} \times \vec{S}_1 \cdot \vec{v}_2 \hat{n} \cdot \vec{a}_1 \hat{n} \cdot \vec{v}_1 - 8 \hat{n} \times \vec{S}_1 \cdot \vec{a}_2 \hat{n} \cdot \vec{a}_1 \hat{n} \cdot \vec{v}_1 + 2 \hat{n} \times \vec{S}_1 \cdot \vec{v}_1 \vec{a}_1 \cdot \vec{a}_2 + \right. \\ \left. 2 \hat{n} \times \vec{S}_1 \cdot \vec{v}_1 \vec{a}_1 \cdot \vec{v}_2 + 2 \hat{n} \times \vec{S}_1 \cdot \vec{a}_1 \vec{v}_1 \cdot \vec{a}_2 + 2 \hat{n} \times \vec{S}_1 \cdot \vec{a}_1 \vec{v}_1 \cdot \vec{v}_2 \right) m_1 m_2 G^2 + \frac{1}{r^2} \\ \left( -4 \hat{n} \times \vec{S}_1 \cdot \vec{v}_2 (\hat{n} \cdot \vec{v}_1)^3 - 4 \hat{n} \times \vec{S}_1 \cdot \vec{a}_2 (\hat{n} \cdot \vec{v}_1)^3 - 2 \vec{S}_1 \times \vec{v}_1 \cdot \vec{v}_2 (\hat{n} \cdot \vec{v}_1)^2 + 4 \vec{S}_1 \times \vec{a}_1 \cdot \vec{v}_2 (\hat{n} \cdot \vec{v}_1)^2 - \right. \\ \left. 2 \vec{S}_1 \times \vec{v}_1 \cdot \vec{a}_2 (\hat{n} \cdot \vec{v}_1)^2 + 40 \hat{n} \times \vec{S}_1 \cdot \vec{v}_2 \hat{n} \cdot \vec{a}_1 (\hat{n} \cdot \vec{v}_1)^2 + 8 \vec{S}_1 \times \vec{v}_1 \cdot \vec{v}_2 \hat{n} \cdot \vec{a}_1 \hat{n} \cdot \vec{v}_1 - 32 \hat{n} \times \vec{S}_1 \cdot \vec{v}_2 \hat{n} \cdot \vec{a}_1 \hat{n} \cdot \vec{v}_2 \hat{n} \cdot \vec{v}_1 - \right. \\ \left. 3 \hat{n} \times \vec{S}_1 \cdot \vec{v}_1 \vec{a}_1 \cdot \vec{v}_2 \hat{n} \cdot \vec{v}_1 + 8 \hat{n} \times \vec{S}_1 \cdot \vec{v}_2 \vec{a}_1 \cdot \vec{v}_2 \hat{n} \cdot \vec{v}_1 - 5 \hat{n} \times \vec{S}_1 \cdot \vec{v}_2 \vec{v}_1 \cdot \vec{a}_1 \hat{n} \cdot \vec{v}_1 + 2 \hat{n} \times \vec{S}_1 \cdot \vec{v}_1 \vec{v}_1 \cdot \vec{a}_2 \hat{n} \cdot \vec{v}_1 - \right. \\ \left. 2 \hat{n} \times \vec{S}_1 \cdot \vec{v}_2 \vec{v}_1 \cdot \vec{v}_1 \hat{n} \cdot \vec{v}_1 - 2 \hat{n} \times \vec{S}_1 \cdot \vec{a}_2 \vec{v}_1 \cdot \vec{v}_1 \hat{n} \cdot \vec{v}_1 + 2 \hat{n} \times \vec{S}_1 \cdot \vec{v}_1 \vec{v}_1 \cdot \vec{v}_2 \hat{n} \cdot \vec{v}_1 - 9 \hat{n} \times \vec{S}_1 \cdot \vec{a}_1 \vec{v}_1 \cdot \vec{v}_2 \hat{n} \cdot \vec{v}_1 - \right. \\ \left. 2 \vec{S}_1 \times \vec{v}_1 \cdot \vec{v}_2 \vec{a}_1 \cdot \vec{v}_2 + 4 \hat{n} \times \vec{S}_1 \cdot \vec{v}_1 \hat{n} \cdot \vec{v}_2 \vec{a}_1 \cdot \vec{v}_2 + 2 \vec{S}_1 \times \vec{v}_1 \cdot \vec{v}_2 \vec{v}_1 \cdot \vec{a}_1 - 3 \hat{n} \times \vec{S}_1 \cdot \vec{v}_1 \hat{n} \cdot \vec{v}_2 \vec{v}_1 \cdot \vec{a}_1 - \right. \\ \left. 2 \vec{S}_1 \times \vec{a}_1 \cdot \vec{v}_2 \vec{v}_1 \cdot \vec{v}_1 - 7 \hat{n} \times \vec{S}_1 \cdot \vec{v}_2 \hat{n} \cdot \vec{a}_1 \vec{v}_1 \cdot \vec{v}_1 + 3 \hat{n} \times \vec{S}_1 \cdot \vec{a}_1 \hat{n} \cdot \vec{v}_2 \vec{v}_1 \cdot \vec{v}_1 - 2 \vec{S}_1 \times \vec{a}_1 \cdot \vec{v}_2 \vec{v}_1 \cdot \vec{v}_2 - \right. \\ \left. 3 \vec{S}_1 \times \vec{v}_1 \cdot \vec{a}_1 \vec{v}_1 \cdot \vec{v}_2 + 8 \hat{n} \times \vec{S}_1 \cdot \vec{v}_2 \hat{n} \cdot \vec{a}_1 \vec{v}_1 \cdot \vec{v}_2 + 4 \hat{n} \times \vec{S}_1 \cdot \vec{a}_1 \hat{n} \cdot \vec{v}_2 \vec{v}_1 \cdot \vec{v}_2 \right) m_1 m_2 G^2 + \frac{1}{r^3} \\ \left( 20 \hat{n} \times \vec{S}_1 \cdot \vec{v}_2 (\hat{n} \cdot \vec{v}_1)^4 + \frac{28}{3} \vec{S}_1 \times \vec{v}_1 \cdot \vec{v}_2 (\hat{n} \cdot \vec{v}_1)^3 - 24 \hat{n} \times \vec{S}_1 \cdot \vec{v}_2 \hat{n} \cdot \vec{v}_2 (\hat{n} \cdot \vec{v}_1)^3 - 8 \vec{S}_1 \times \vec{v}_1 \cdot \vec{v}_2 \hat{n} \cdot \vec{v}_2 (\hat{n} \cdot \vec{v}_1)^2 + \right. \\ \left. 4 \hat{n} \times \vec{S}_1 \cdot \vec{v}_2 \vec{v}_1 \cdot \vec{v}_1 (\hat{n} \cdot \vec{v}_1)^2 - 6 \hat{n} \times \vec{S}_1 \cdot \vec{v}_1 \vec{v}_1 \cdot \vec{v}_2 (\hat{n} \cdot \vec{v}_1)^2 + 12 \hat{n} \times \vec{S}_1 \cdot \vec{v}_2 \vec{v}_1 \cdot \vec{v}_2 (\hat{n} \cdot \vec{v}_1)^2 + \right. \\ \left. 2 \vec{S}_1 \times \vec{v}_1 \cdot \vec{v}_2 \vec{v}_1 \cdot \vec{v}_1 \hat{n} \cdot \vec{v}_1 - 8 \hat{n} \times \vec{S}_1 \cdot \vec{v}_2 \hat{n} \cdot \vec{v}_2 \vec{v}_1 \cdot \vec{v}_1 \hat{n} \cdot \vec{v}_1 + 2 \vec{S}_1 \times \vec{v}_1 \cdot \vec{v}_2 \vec{v}_1 \cdot \vec{v}_2 \hat{n} \cdot \vec{v}_1 + \right. \\ \left. 8 \hat{n} \times \vec{S}_1 \cdot \vec{v}_1 \hat{n} \cdot \vec{v}_2 \vec{v}_1 \cdot \vec{v}_2 \hat{n} \cdot \vec{v}_1 - 2 \hat{n} \times \vec{S}_1 \cdot \vec{v}_2 (\vec{v}_1 \cdot \vec{v}_1)^2 - 2 \hat{n} \times \vec{S}_1 \cdot \vec{v}_1 (\vec{v}_1 \cdot \vec{v}_2)^2 + 2 \hat{n} \times \vec{S}_1 \cdot \vec{v}_2 \vec{v}_1 \cdot \vec{v}_1 \vec{v}_1 \cdot \vec{v}_2 \right) m_1 m_2 G^2 \}$$

{DiagSet[2, 2, 17],

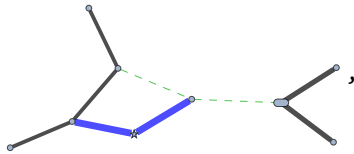

$$\frac{1}{r} G^2 \left( -\frac{8}{3} \vec{a}_2 \times \vec{S}_1 \cdot \vec{v}_2 \hat{n} \cdot \vec{a}_2 - \frac{16}{3} \hat{n} \times \vec{S}_1 \cdot \vec{v}_2 \hat{n} \cdot \vec{v}_2 \hat{n} \cdot \vec{a}_2 + \frac{16}{3} \hat{n} \times \vec{a}_2 \cdot \vec{S}_1 \hat{n} \cdot \vec{v}_2 \hat{n} \cdot \vec{a}_2 + \frac{8}{3} \vec{a}_2 \times \vec{S}_1 \cdot \vec{v}_2 \hat{n} \cdot \vec{v}_2 + \right. \\ \left. 4 \hat{n} \times \vec{S}_1 \cdot \vec{v}_2 \vec{a}_2 \cdot \vec{a}_2 - \frac{4}{3} \hat{n} \times \vec{S}_1 \cdot \vec{v}_2 \vec{a}_2 \cdot \vec{v}_2 + \frac{4}{3} \hat{n} \times \vec{a}_2 \cdot \vec{S}_1 \vec{a}_2 \cdot \vec{v}_2 - 4 \hat{n} \times \vec{a}_2 \cdot \vec{S}_1 \vec{v}_2 \cdot \vec{v}_2 \right) m_2^2 + \frac{1}{r^2} \\ G^2 \left( \frac{16}{3} \hat{n} \times \vec{S}_1 \cdot \vec{v}_2 (\hat{n} \cdot \vec{v}_2)^3 - \frac{16}{3} \hat{n} \times \vec{a}_2 \cdot \vec{S}_1 (\hat{n} \cdot \vec{v}_2)^3 + 12 \vec{a}_2 \times \vec{S}_1 \cdot \vec{v}_2 (\hat{n} \cdot \vec{v}_2)^2 - 32 \hat{n} \times \vec{S}_1 \cdot \vec{v}_2 \hat{n} \cdot \vec{a}_2 (\hat{n} \cdot \vec{v}_2)^2 + \right. \\ \left. \frac{16}{3} \vec{S}_1 \times \vec{v}_1 \cdot \vec{v}_2 \hat{n} \cdot \vec{a}_2 \hat{n} \cdot \vec{v}_2 - \frac{16}{3} \vec{a}_2 \times \vec{S}_1 \cdot \vec{v}_2 \hat{n} \cdot \vec{v}_1 \hat{n} \cdot \vec{v}_2 + \frac{64}{3} \hat{n} \times \vec{S}_1 \cdot \vec{v}_2 \hat{n} \cdot \vec{a}_2 \hat{n} \cdot \vec{v}_1 \hat{n} \cdot \vec{v}_2 - \right. \\ \left. \frac{16}{3} \hat{n} \times \vec{S}_1 \cdot \vec{v}_2 \vec{a}_2 \cdot \vec{v}_1 \hat{n} \cdot \vec{v}_2 + 4 \hat{n} \times \vec{S}_1 \cdot \vec{v}_2 \vec{a}_2 \cdot \vec{v}_2 \hat{n} \cdot \vec{v}_2 - 8 \hat{n} \times \vec{a}_2 \cdot \vec{S}_1 \vec{v}_2 \cdot \vec{v}_2 \hat{n} \cdot \vec{v}_2 + \right. \\ \left. \frac{4}{3} \vec{S}_1 \times \vec{v}_1 \cdot \vec{v}_2 \vec{a}_2 \cdot \vec{v}_2 + \frac{8}{3} \hat{n} \times \vec{S}_1 \cdot \vec{v}_2 \hat{n} \cdot \vec{v}_1 \vec{a}_2 \cdot \vec{v}_2 + \frac{8}{3} \vec{a}_2 \times \vec{S}_1 \cdot \vec{v}_2 \vec{v}_1 \cdot \vec{v}_2 - \frac{16}{3} \hat{n} \times \vec{S}_1 \cdot \vec{v}_2 \hat{n} \cdot \vec{a}_2 \vec{v}_1 \cdot \vec{v}_2 - \right. \\ \left. 4 \vec{a}_2 \times \vec{S}_1 \cdot \vec{v}_1 \vec{v}_2 \cdot \vec{v}_2 + 2 \vec{a}_2 \times \vec{S}_1 \cdot \vec{v}_2 \vec{v}_2 \cdot \vec{v}_2 + 4 \hat{n} \times \vec{S}_1 \cdot \vec{v}_2 \hat{n} \cdot \vec{a}_2 \vec{v}_2 \cdot \vec{v}_2 + 8 \hat{n} \times \vec{a}_2 \cdot \vec{S}_1 \hat{n} \cdot \vec{v}_1 \vec{v}_2 \cdot \vec{v}_2 \right) m_2^2 + \\ \frac{1}{r^3} G^2 \left( 24 \hat{n} \times \vec{S}_1 \cdot \vec{v}_2 (\hat{n} \cdot \vec{v}_2)^4 - \frac{16}{3} \vec{S}_1 \times \vec{v}_1 \cdot \vec{v}_2 (\hat{n} \cdot \vec{v}_2)^3 - 32 \hat{n} \times \vec{S}_1 \cdot \vec{v}_2 \hat{n} \cdot \vec{v}_1 (\hat{n} \cdot \vec{v}_2)^3 + \right. \\ \left. 16 \hat{n} \times \vec{S}_1 \cdot \vec{v}_2 \vec{v}_1 \cdot \vec{v}_2 (\hat{n} \cdot \vec{v}_2)^2 - 4 \hat{n} \times \vec{S}_1 \cdot \vec{v}_2 \vec{v}_2 \cdot \vec{v}_2 (\hat{n} \cdot \vec{v}_2)^2 - 2 \hat{n} \times \vec{S}_1 \cdot \vec{v}_2 (\vec{v}_2 \cdot \vec{v}_2)^2 \right) m_2^2 \}$$

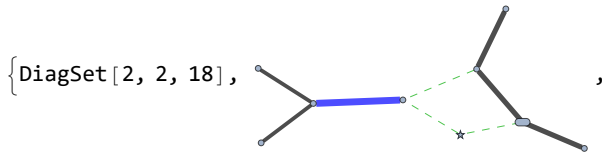

$$\begin{aligned} & \frac{1}{r} \left( -\frac{1}{3} \hat{n} \times \vec{S}_1 \cdot \vec{a}_1 (\hat{n} \cdot \vec{v}_2)^2 + \frac{10}{3} \vec{S}_1 \times \vec{a}_1 \cdot \vec{v}_2 \hat{n} \cdot \vec{v}_2 + \frac{10}{3} \vec{S}_1 \times \vec{v}_1 \cdot \vec{a}_2 \hat{n} \cdot \vec{v}_2 - \frac{2}{3} \hat{n} \times \vec{S}_1 \cdot \vec{v}_1 \hat{n} \cdot \vec{a}_2 \hat{n} \cdot \vec{v}_2 + \frac{10}{3} \vec{S}_1 \times \vec{v}_1 \cdot \vec{v}_2 \hat{n} \cdot \vec{a}_2 + \right. \\ & \quad \left. 2 \hat{n} \times \vec{S}_1 \cdot \vec{v}_2 \vec{a}_1 \cdot \vec{v}_2 + 2 \hat{n} \times \vec{S}_1 \cdot \vec{v}_2 \vec{v}_1 \cdot \vec{a}_2 + 2 \hat{n} \times \vec{S}_1 \cdot \vec{a}_2 \vec{v}_1 \cdot \vec{v}_2 - \frac{14}{3} \hat{n} \times \vec{S}_1 \cdot \vec{v}_1 \vec{v}_2 \cdot \vec{a}_2 - \frac{7}{3} \hat{n} \times \vec{S}_1 \cdot \vec{a}_1 \vec{v}_2 \cdot \vec{v}_2 \right) m_1 m_2 G^2 + \\ & \frac{1}{r^2} \left( -\frac{4}{3} \hat{n} \times \vec{S}_1 \cdot \vec{v}_1 (\hat{n} \cdot \vec{v}_2)^3 + 7 \vec{S}_1 \times \vec{v}_1 \cdot \vec{v}_2 (\hat{n} \cdot \vec{v}_2)^2 + \frac{2}{3} \vec{S}_1 \times \vec{v}_1 \cdot \vec{a}_1 (\hat{n} \cdot \vec{v}_2)^2 + \frac{2}{3} \hat{n} \times \vec{S}_1 \cdot \vec{v}_1 \hat{n} \cdot \vec{v}_1 (\hat{n} \cdot \vec{v}_2)^2 + \right. \\ & \quad \frac{2}{3} \hat{n} \times \vec{S}_1 \cdot \vec{a}_1 \hat{n} \cdot \vec{v}_1 (\hat{n} \cdot \vec{v}_2)^2 - \frac{16}{3} \vec{S}_1 \times \vec{v}_1 \cdot \vec{v}_2 \hat{n} \cdot \vec{v}_1 \hat{n} \cdot \vec{v}_2 - \frac{4}{3} \vec{S}_1 \times \vec{a}_1 \cdot \vec{v}_2 \hat{n} \cdot \vec{v}_1 \hat{n} \cdot \vec{v}_2 - \frac{4}{3} \vec{S}_1 \times \vec{v}_1 \cdot \vec{a}_2 \hat{n} \cdot \vec{v}_1 \hat{n} \cdot \vec{v}_2 + \\ & \quad \frac{4}{3} \hat{n} \times \vec{S}_1 \cdot \vec{v}_1 \hat{n} \cdot \vec{a}_2 \hat{n} \cdot \vec{v}_1 \hat{n} \cdot \vec{v}_2 - \hat{n} \times \vec{S}_1 \cdot \vec{v}_1 \vec{a}_1 \cdot \vec{v}_2 \hat{n} \cdot \vec{v}_2 + \hat{n} \times \vec{S}_1 \cdot \vec{v}_2 \vec{v}_1 \cdot \vec{a}_1 \hat{n} \cdot \vec{v}_2 - \frac{4}{3} \hat{n} \times \vec{S}_1 \cdot \vec{v}_1 \vec{v}_1 \cdot \vec{a}_2 \hat{n} \cdot \vec{v}_2 - \\ & \quad \hat{n} \times \vec{S}_1 \cdot \vec{v}_2 \vec{v}_1 \cdot \vec{v}_1 \hat{n} \cdot \vec{v}_2 + \hat{n} \times \vec{S}_1 \cdot \vec{a}_2 \vec{v}_1 \cdot \vec{v}_1 \hat{n} \cdot \vec{v}_2 + \frac{2}{3} \hat{n} \times \vec{S}_1 \cdot \vec{v}_1 \vec{v}_1 \cdot \vec{v}_2 \hat{n} \cdot \vec{v}_2 + 4 \hat{n} \times \vec{S}_1 \cdot \vec{v}_2 \vec{v}_1 \cdot \vec{v}_2 \hat{n} \cdot \vec{v}_2 - \\ & \quad \frac{1}{3} \hat{n} \times \vec{S}_1 \cdot \vec{a}_1 \vec{v}_1 \cdot \vec{v}_2 \hat{n} \cdot \vec{v}_2 - 4 \hat{n} \times \vec{S}_1 \cdot \vec{v}_1 \vec{v}_2 \cdot \vec{v}_2 \hat{n} \cdot \vec{v}_2 - \frac{4}{3} \vec{S}_1 \times \vec{v}_1 \cdot \vec{v}_2 \hat{n} \cdot \vec{a}_2 \hat{n} \cdot \vec{v}_1 - \vec{S}_1 \times \vec{v}_1 \cdot \vec{v}_2 \vec{a}_1 \cdot \vec{v}_2 - \\ & \quad \frac{1}{3} \vec{S}_1 \times \vec{v}_1 \cdot \vec{v}_2 \vec{v}_1 \cdot \vec{a}_2 - \hat{n} \times \vec{S}_1 \cdot \vec{v}_2 \hat{n} \cdot \vec{v}_1 \vec{v}_1 \cdot \vec{a}_2 + \hat{n} \times \vec{S}_1 \cdot \vec{v}_2 \hat{n} \cdot \vec{a}_2 \vec{v}_1 \cdot \vec{v}_1 + \frac{5}{3} \vec{S}_1 \times \vec{v}_1 \cdot \vec{v}_2 \vec{v}_1 \cdot \vec{v}_2 + \\ & \quad \frac{2}{3} \vec{S}_1 \times \vec{a}_1 \cdot \vec{v}_2 \vec{v}_1 \cdot \vec{v}_2 - \frac{1}{3} \vec{S}_1 \times \vec{v}_1 \cdot \vec{a}_2 \vec{v}_1 \cdot \vec{v}_2 - \hat{n} \times \vec{S}_1 \cdot \vec{v}_2 \hat{n} \cdot \vec{a}_1 \vec{v}_1 \cdot \vec{v}_2 - \frac{4}{3} \hat{n} \times \vec{S}_1 \cdot \vec{v}_1 \hat{n} \cdot \vec{a}_2 \vec{v}_1 \cdot \vec{v}_2 - \\ & \quad 3 \hat{n} \times \vec{S}_1 \cdot \vec{v}_2 \hat{n} \cdot \vec{v}_1 \vec{v}_1 \cdot \vec{v}_2 - \hat{n} \times \vec{S}_1 \cdot \vec{a}_2 \hat{n} \cdot \vec{v}_1 \vec{v}_1 \cdot \vec{v}_2 + \frac{8}{3} \hat{n} \times \vec{S}_1 \cdot \vec{v}_1 \hat{n} \cdot \vec{v}_1 \vec{v}_2 \cdot \vec{a}_2 - \frac{1}{3} \vec{S}_1 \times \vec{v}_1 \cdot \vec{v}_2 \vec{v}_2 \cdot \vec{v}_2 + \\ & \quad \frac{2}{3} \vec{S}_1 \times \vec{v}_1 \cdot \vec{a}_1 \vec{v}_2 \cdot \vec{v}_2 + \hat{n} \times \vec{S}_1 \cdot \vec{v}_1 \hat{n} \cdot \vec{a}_1 \vec{v}_2 \cdot \vec{v}_2 + \frac{10}{3} \hat{n} \times \vec{S}_1 \cdot \vec{v}_1 \hat{n} \cdot \vec{v}_1 \vec{v}_2 \cdot \vec{v}_2 + \frac{1}{3} \hat{n} \times \vec{S}_1 \cdot \vec{a}_1 \hat{n} \cdot \vec{v}_1 \vec{v}_2 \cdot \vec{v}_2 \Big) m_1 m_2 G^2 + \\ & \frac{1}{r^3} \left( 4 \hat{n} \times \vec{S}_1 \cdot \vec{v}_1 \hat{n} \cdot \vec{v}_1 (\hat{n} \cdot \vec{v}_2)^3 - \frac{3}{2} \hat{n} \times \vec{S}_1 \cdot \vec{v}_1 (\hat{n} \cdot \vec{v}_1)^2 (\hat{n} \cdot \vec{v}_2)^2 - 6 \vec{S}_1 \times \vec{v}_1 \cdot \vec{v}_2 \hat{n} \cdot \vec{v}_1 (\hat{n} \cdot \vec{v}_2)^2 - \right. \\ & \quad \frac{1}{2} \hat{n} \times \vec{S}_1 \cdot \vec{v}_1 \vec{v}_1 \cdot \vec{v}_1 (\hat{n} \cdot \vec{v}_2)^2 + 4 \hat{n} \times \vec{S}_1 \cdot \vec{v}_2 \vec{v}_1 \cdot \vec{v}_1 (\hat{n} \cdot \vec{v}_2)^2 - 6 \hat{n} \times \vec{S}_1 \cdot \vec{v}_1 \vec{v}_1 \cdot \vec{v}_2 (\hat{n} \cdot \vec{v}_2)^2 + \\ & \quad 3 \vec{S}_1 \times \vec{v}_1 \cdot \vec{v}_2 (\hat{n} \cdot \vec{v}_1)^2 \hat{n} \cdot \vec{v}_2 - 2 \vec{S}_1 \times \vec{v}_1 \cdot \vec{v}_2 \vec{v}_1 \cdot \vec{v}_1 \hat{n} \cdot \vec{v}_2 + 2 \vec{S}_1 \times \vec{v}_1 \cdot \vec{v}_2 \vec{v}_1 \cdot \vec{v}_2 \hat{n} \cdot \vec{v}_2 + \\ & \quad 2 \hat{n} \times \vec{S}_1 \cdot \vec{v}_1 \hat{n} \cdot \vec{v}_1 \vec{v}_1 \cdot \vec{v}_2 \hat{n} \cdot \vec{v}_2 - 4 \hat{n} \times \vec{S}_1 \cdot \vec{v}_2 \hat{n} \cdot \vec{v}_1 \vec{v}_1 \cdot \vec{v}_2 \hat{n} \cdot \vec{v}_2 + 4 \hat{n} \times \vec{S}_1 \cdot \vec{v}_1 \hat{n} \cdot \vec{v}_1 \vec{v}_2 \cdot \vec{v}_2 \hat{n} \cdot \vec{v}_2 - \\ & \quad \hat{n} \times \vec{S}_1 \cdot \vec{v}_1 (\vec{v}_1 \cdot \vec{v}_2)^2 + \hat{n} \times \vec{S}_1 \cdot \vec{v}_2 (\vec{v}_1 \cdot \vec{v}_2)^2 + 2 \hat{n} \times \vec{S}_1 \cdot \vec{v}_2 (\hat{n} \cdot \vec{v}_1)^2 \vec{v}_1 \cdot \vec{v}_2 + \vec{S}_1 \times \vec{v}_1 \cdot \vec{v}_2 \hat{n} \cdot \vec{v}_1 \vec{v}_1 \cdot \vec{v}_2 - \\ & \quad \left. \frac{5}{2} \hat{n} \times \vec{S}_1 \cdot \vec{v}_1 (\hat{n} \cdot \vec{v}_1)^2 \vec{v}_2 \cdot \vec{v}_2 + \frac{3}{2} \hat{n} \times \vec{S}_1 \cdot \vec{v}_1 \vec{v}_1 \cdot \vec{v}_1 \vec{v}_2 \cdot \vec{v}_2 - \hat{n} \times \vec{S}_1 \cdot \vec{v}_2 \vec{v}_1 \cdot \vec{v}_1 \vec{v}_2 \cdot \vec{v}_2 \right) m_1 m_2 G^2 \Big\} \end{aligned}$$

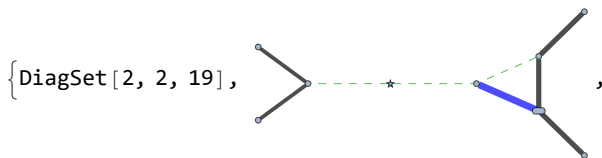

$$\begin{aligned} & \frac{1}{r} \left( -(\vec{S}_1 \times \vec{v}_1 \cdot \vec{a}_2) \hat{n} \cdot \vec{a}_1 - \vec{S}_1 \times \vec{v}_1 \cdot \vec{a}_2 \hat{n} \cdot \vec{v}_1 - \vec{S}_1 \times \vec{a}_1 \cdot \vec{a}_2 \hat{n} \cdot \vec{v}_1 + 4 \hat{n} \times \vec{S}_1 \cdot \vec{v}_1 \vec{a}_1 \cdot \vec{a}_2 - \right. \\ & \quad \left. 6 \hat{n} \times \vec{S}_1 \cdot \vec{a}_2 \vec{v}_1 \cdot \vec{a}_1 + 4 \hat{n} \times \vec{S}_1 \cdot \vec{v}_1 \vec{v}_1 \cdot \vec{a}_2 + 4 \hat{n} \times \vec{S}_1 \cdot \vec{a}_1 \vec{v}_1 \cdot \vec{a}_2 - 3 \hat{n} \times \vec{S}_1 \cdot \vec{a}_2 \vec{v}_1 \cdot \vec{v}_1 \right) m_1 m_2 G^2 + \frac{1}{r^2} \\ & \left( 2 \vec{S}_1 \times \vec{v}_1 \cdot \vec{a}_2 (\hat{n} \cdot \vec{v}_1)^2 - 2 \vec{S}_1 \times \vec{v}_1 \cdot \vec{v}_2 \hat{n} \cdot \vec{v}_2 \hat{n} \cdot \vec{v}_1 - 2 \vec{S}_1 \times \vec{a}_1 \cdot \vec{v}_2 \hat{n} \cdot \vec{v}_2 \hat{n} \cdot \vec{v}_1 - 8 \hat{n} \times \vec{S}_1 \cdot \vec{v}_1 \vec{v}_1 \cdot \vec{a}_2 \hat{n} \cdot \vec{v}_1 + \right. \\ & \quad 6 \hat{n} \times \vec{S}_1 \cdot \vec{a}_2 \vec{v}_1 \cdot \vec{v}_1 \hat{n} \cdot \vec{v}_1 - 2 \vec{S}_1 \times \vec{v}_1 \cdot \vec{v}_2 \hat{n} \cdot \vec{a}_1 \hat{n} \cdot \vec{v}_2 - 3 \vec{S}_1 \times \vec{v}_1 \cdot \vec{v}_2 \vec{a}_1 \cdot \vec{v}_2 + 8 \hat{n} \times \vec{S}_1 \cdot \vec{v}_1 \hat{n} \cdot \vec{v}_2 \vec{a}_1 \cdot \vec{v}_2 - \\ & \quad \left. 12 \hat{n} \times \vec{S}_1 \cdot \vec{v}_2 \hat{n} \cdot \vec{v}_2 \vec{v}_1 \cdot \vec{a}_1 + 2 \vec{S}_1 \times \vec{v}_1 \cdot \vec{a}_2 \vec{v}_1 \cdot \vec{v}_1 - 6 \hat{n} \times \vec{S}_1 \cdot \vec{v}_2 \hat{n} \cdot \vec{v}_2 \vec{v}_1 \cdot \vec{v}_1 - 3 \vec{S}_1 \times \vec{v}_1 \cdot \vec{v}_2 \vec{v}_1 \cdot \vec{v}_2 - \right. \end{aligned}$$

$$\left. 3 \vec{S}_1 \times \vec{a}_1 \cdot \vec{v}_2 \vec{v}_1 \cdot \vec{v}_2 + 8 \hat{n} \times \vec{S}_1 \cdot \vec{v}_1 \hat{n} \cdot \vec{v}_2 \vec{v}_1 \cdot \vec{v}_2 + 8 \hat{n} \times \vec{S}_1 \cdot \vec{a}_1 \hat{n} \cdot \vec{v}_2 \vec{v}_1 \cdot \vec{v}_2 \right) m_1 m_2 G^2 + \frac{1}{r^3} \\ \left( 8 \vec{S}_1 \times \vec{v}_1 \cdot \vec{v}_2 \hat{n} \cdot \vec{v}_2 (\hat{n} \cdot \vec{v}_1)^2 + 24 \hat{n} \times \vec{S}_1 \cdot \vec{v}_2 \hat{n} \cdot \vec{v}_2 \vec{v}_1 \cdot \vec{v}_1 \hat{n} \cdot \vec{v}_1 + 4 \vec{S}_1 \times \vec{v}_1 \cdot \vec{v}_2 \vec{v}_1 \cdot \vec{v}_2 \hat{n} \cdot \vec{v}_1 - 32 \hat{n} \times \vec{S}_1 \cdot \vec{v}_1 \right. \\ \left. \hat{n} \cdot \vec{v}_2 \vec{v}_1 \cdot \vec{v}_2 \hat{n} \cdot \vec{v}_1 + 8 \hat{n} \times \vec{S}_1 \cdot \vec{v}_1 (\vec{v}_1 \cdot \vec{v}_2)^2 + 4 \vec{S}_1 \times \vec{v}_1 \cdot \vec{v}_2 \hat{n} \cdot \vec{v}_2 \vec{v}_1 \cdot \vec{v}_1 - 6 \hat{n} \times \vec{S}_1 \cdot \vec{v}_2 \vec{v}_1 \cdot \vec{v}_1 \vec{v}_1 \cdot \vec{v}_2 \right) m_1 m_2 G^2 \Big\}$$

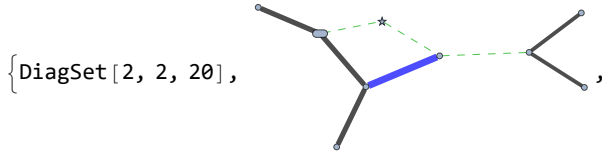

$$\frac{1}{r} \left( \frac{4}{3} \hat{n} \times \vec{S}_1 \cdot \vec{a}_2 (\hat{n} \cdot \vec{v}_1)^2 + \frac{16}{3} \vec{S}_1 \times \vec{a}_1 \cdot \vec{v}_2 \hat{n} \cdot \vec{v}_1 + \frac{16}{3} \vec{S}_1 \times \vec{v}_1 \cdot \vec{a}_2 \hat{n} \cdot \vec{v}_1 + \frac{8}{3} \hat{n} \times \vec{S}_1 \cdot \vec{v}_2 \hat{n} \cdot \vec{a}_1 \hat{n} \cdot \vec{v}_1 + \frac{16}{3} \vec{S}_1 \times \vec{v}_1 \cdot \vec{v}_2 \hat{n} \cdot \vec{a}_1 - \right. \\ \left. 6 \hat{n} \times \vec{S}_1 \cdot \vec{v}_1 \vec{a}_1 \cdot \vec{v}_2 + \frac{32}{3} \hat{n} \times \vec{S}_1 \cdot \vec{v}_2 \vec{v}_1 \cdot \vec{a}_1 - 6 \hat{n} \times \vec{S}_1 \cdot \vec{v}_1 \vec{v}_1 \cdot \vec{a}_2 + \frac{16}{3} \hat{n} \times \vec{S}_1 \cdot \vec{a}_2 \vec{v}_1 \cdot \vec{v}_1 - 6 \hat{n} \times \vec{S}_1 \cdot \vec{a}_1 \vec{v}_1 \cdot \vec{v}_2 \right) m_1 m_2 G^2 + \\ \frac{1}{r^2} \left( -\frac{4}{3} \hat{n} \times \vec{S}_1 \cdot \vec{v}_2 (\hat{n} \cdot \vec{v}_1)^3 - 4 \hat{n} \times \vec{S}_1 \cdot \vec{a}_2 (\hat{n} \cdot \vec{v}_1)^3 - 6 \vec{S}_1 \times \vec{v}_1 \cdot \vec{v}_2 (\hat{n} \cdot \vec{v}_1)^2 - 4 \vec{S}_1 \times \vec{a}_1 \cdot \vec{v}_2 (\hat{n} \cdot \vec{v}_1)^2 - \right. \\ \left. 6 \vec{S}_1 \times \vec{v}_1 \cdot \vec{a}_2 (\hat{n} \cdot \vec{v}_1)^2 - 8 \hat{n} \times \vec{S}_1 \cdot \vec{v}_2 \hat{n} \cdot \vec{a}_1 (\hat{n} \cdot \vec{v}_1)^2 + \frac{16}{3} \hat{n} \times \vec{S}_1 \cdot \vec{v}_2 \hat{n} \cdot \vec{v}_2 (\hat{n} \cdot \vec{v}_1)^2 - \right. \\ \left. 8 \vec{S}_1 \times \vec{v}_1 \cdot \vec{v}_2 \hat{n} \cdot \vec{a}_1 \hat{n} \cdot \vec{v}_1 + \frac{32}{3} \vec{S}_1 \times \vec{v}_1 \cdot \vec{v}_2 \hat{n} \cdot \vec{v}_2 \hat{n} \cdot \vec{v}_1 + 7 \hat{n} \times \vec{S}_1 \cdot \vec{v}_1 \vec{a}_1 \cdot \vec{v}_2 \hat{n} \cdot \vec{v}_1 - 7 \hat{n} \times \vec{S}_1 \cdot \vec{v}_2 \vec{v}_1 \cdot \vec{a}_1 \hat{n} \cdot \vec{v}_1 + \right. \\ \left. 6 \hat{n} \times \vec{S}_1 \cdot \vec{v}_1 \vec{v}_1 \cdot \vec{a}_2 \hat{n} \cdot \vec{v}_1 - 6 \hat{n} \times \vec{S}_1 \cdot \vec{v}_2 \vec{v}_1 \cdot \vec{v}_1 \hat{n} \cdot \vec{v}_1 - 2 \hat{n} \times \vec{S}_1 \cdot \vec{a}_2 \vec{v}_1 \cdot \vec{v}_1 \hat{n} \cdot \vec{v}_1 + 6 \hat{n} \times \vec{S}_1 \cdot \vec{v}_1 \vec{v}_1 \cdot \vec{v}_2 \hat{n} \cdot \vec{v}_1 - \right. \\ \left. \frac{8}{3} \hat{n} \times \vec{S}_1 \cdot \vec{v}_2 \vec{v}_1 \cdot \vec{v}_2 \hat{n} \cdot \vec{v}_1 + 5 \hat{n} \times \vec{S}_1 \cdot \vec{a}_1 \vec{v}_1 \cdot \vec{v}_2 \hat{n} \cdot \vec{v}_1 - 2 \vec{S}_1 \times \vec{v}_1 \cdot \vec{v}_2 \vec{v}_1 \cdot \vec{a}_1 - \hat{n} \times \vec{S}_1 \cdot \vec{v}_1 \hat{n} \cdot \vec{v}_2 \vec{v}_1 \cdot \vec{a}_1 + \right. \\ \left. 2 \vec{S}_1 \times \vec{a}_1 \cdot \vec{v}_2 \vec{v}_1 \cdot \vec{v}_1 + 3 \hat{n} \times \vec{S}_1 \cdot \vec{v}_2 \hat{n} \cdot \vec{a}_1 \vec{v}_1 \cdot \vec{v}_1 + \frac{32}{3} \hat{n} \times \vec{S}_1 \cdot \vec{v}_2 \hat{n} \cdot \vec{v}_2 \vec{v}_1 \cdot \vec{v}_1 + \hat{n} \times \vec{S}_1 \cdot \vec{a}_1 \hat{n} \cdot \vec{v}_2 \vec{v}_1 \cdot \vec{v}_1 + \right. \\ \left. \frac{2}{3} \vec{S}_1 \times \vec{v}_1 \cdot \vec{v}_2 \vec{v}_1 \cdot \vec{v}_2 + 3 \vec{S}_1 \times \vec{v}_1 \cdot \vec{a}_1 \vec{v}_1 \cdot \vec{v}_2 - 12 \hat{n} \times \vec{S}_1 \cdot \vec{v}_1 \hat{n} \cdot \vec{v}_2 \vec{v}_1 \cdot \vec{v}_2 \right) m_1 m_2 G^2 + \frac{1}{r^3} \\ \left( 4 \hat{n} \times \vec{S}_1 \cdot \vec{v}_2 (\hat{n} \cdot \vec{v}_1)^4 + \frac{20}{3} \vec{S}_1 \times \vec{v}_1 \cdot \vec{v}_2 (\hat{n} \cdot \vec{v}_1)^3 - 24 \hat{n} \times \vec{S}_1 \cdot \vec{v}_2 \hat{n} \cdot \vec{v}_2 (\hat{n} \cdot \vec{v}_1)^3 - 24 \vec{S}_1 \times \vec{v}_1 \cdot \vec{v}_2 \hat{n} \cdot \vec{v}_2 (\hat{n} \cdot \vec{v}_1)^2 + \right. \\ \left. 4 \hat{n} \times \vec{S}_1 \cdot \vec{v}_2 \vec{v}_1 \cdot \vec{v}_1 (\hat{n} \cdot \vec{v}_1)^2 - 6 \hat{n} \times \vec{S}_1 \cdot \vec{v}_1 \vec{v}_1 \cdot \vec{v}_2 (\hat{n} \cdot \vec{v}_1)^2 + 12 \hat{n} \times \vec{S}_1 \cdot \vec{v}_2 \vec{v}_1 \cdot \vec{v}_2 (\hat{n} \cdot \vec{v}_1)^2 - 2 \vec{S}_1 \times \vec{v}_1 \cdot \vec{v}_2 \right. \\ \left. \vec{v}_1 \cdot \vec{v}_1 \hat{n} \cdot \vec{v}_1 - 8 \hat{n} \times \vec{S}_1 \cdot \vec{v}_2 \hat{n} \cdot \vec{v}_2 \vec{v}_1 \cdot \vec{v}_1 \hat{n} \cdot \vec{v}_1 + 6 \vec{S}_1 \times \vec{v}_1 \cdot \vec{v}_2 \vec{v}_1 \cdot \vec{v}_2 \hat{n} \cdot \vec{v}_1 + 24 \hat{n} \times \vec{S}_1 \cdot \vec{v}_1 \hat{n} \cdot \vec{v}_2 \vec{v}_1 \cdot \vec{v}_2 \hat{n} \cdot \vec{v}_1 - \right. \\ \left. 2 \hat{n} \times \vec{S}_1 \cdot \vec{v}_2 (\vec{v}_1 \cdot \vec{v}_1)^2 - 6 \hat{n} \times \vec{S}_1 \cdot \vec{v}_1 (\vec{v}_1 \cdot \vec{v}_2)^2 + 2 \hat{n} \times \vec{S}_1 \cdot \vec{v}_1 \vec{v}_1 \cdot \vec{v}_1 \vec{v}_1 \cdot \vec{v}_2 + 2 \hat{n} \times \vec{S}_1 \cdot \vec{v}_2 \vec{v}_1 \cdot \vec{v}_1 \vec{v}_1 \cdot \vec{v}_2 \right) m_1 m_2 G^2 \Big\}$$

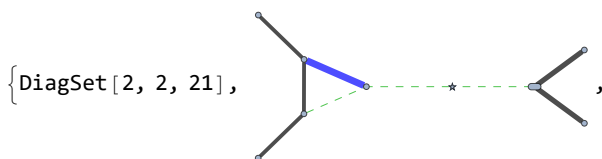

$$\frac{1}{r^2} G^2 m_2^2 \left( -\frac{8}{3} (\hat{n} \cdot \vec{v}_2)^2 \vec{a}_2 \times \vec{S}_1 \cdot \vec{v}_1 + \frac{32}{3} \hat{n} \cdot \vec{v}_1 (\hat{n} \cdot \vec{v}_2)^2 \hat{n} \times \vec{a}_2 \cdot \vec{S}_1 - \frac{16}{3} \hat{n} \cdot \vec{a}_2 \hat{n} \cdot \vec{v}_2 \vec{S}_1 \times \vec{v}_1 \cdot \vec{v}_2 - \right. \\ \left. \frac{64}{3} \hat{n} \cdot \vec{a}_2 \hat{n} \cdot \vec{v}_1 \hat{n} \cdot \vec{v}_2 \hat{n} \times \vec{S}_1 \cdot \vec{v}_2 + \frac{16}{3} \vec{a}_2 \cdot \vec{v}_1 \hat{n} \cdot \vec{v}_2 \hat{n} \times \vec{S}_1 \cdot \vec{v}_2 - \frac{16}{3} \vec{v}_1 \cdot \vec{v}_2 \hat{n} \cdot \vec{v}_2 \hat{n} \times \vec{a}_2 \cdot \vec{S}_1 + \right. \\ \left. \frac{16}{3} \vec{a}_2 \cdot \vec{v}_2 \hat{n} \cdot \vec{v}_1 \hat{n} \times \vec{S}_1 \cdot \vec{v}_2 + \frac{16}{3} \vec{v}_1 \cdot \vec{v}_2 \hat{n} \cdot \vec{a}_2 \hat{n} \times \vec{S}_1 \cdot \vec{v}_2 - \frac{8}{3} \vec{v}_2 \cdot \vec{v}_2 \hat{n} \cdot \vec{v}_1 \hat{n} \times \vec{a}_2 \cdot \vec{S}_1 + \right. \\ \left. \frac{8}{3} \vec{a}_2 \cdot \vec{v}_2 \vec{S}_1 \times \vec{v}_1 \cdot \vec{v}_2 + \frac{4}{3} \vec{v}_2 \cdot \vec{v}_2 \vec{a}_2 \times \vec{S}_1 \cdot \vec{v}_1 + \frac{32}{3} (\hat{n} \cdot \vec{v}_2)^3 \hat{n} \times \vec{S}_1 \cdot \vec{v}_2 - 8 \vec{v}_2 \cdot \vec{v}_2 \hat{n} \cdot \vec{v}_2 \hat{n} \times \vec{S}_1 \cdot \vec{v}_2 \right) + \frac{1}{r} \\ G^2 m_2^2 \left( -\frac{8}{3} (\hat{n} \cdot \vec{v}_2)^2 \hat{n} \times \vec{a}_2 \cdot \vec{S}_1 + \frac{16}{3} \hat{n} \cdot \vec{a}_2 \hat{n} \cdot \vec{v}_2 \hat{n} \times \vec{S}_1 \cdot \vec{v}_2 - \frac{8}{3} \vec{a}_2 \cdot \vec{v}_2 \hat{n} \times \vec{S}_1 \cdot \vec{v}_2 + \frac{4}{3} \vec{v}_2 \cdot \vec{v}_2 \hat{n} \times \vec{a}_2 \cdot \vec{S}_1 \right) + \\ \frac{1}{r^3} G^2 m_2^2 \left( -\frac{32}{3} (\hat{n} \cdot \vec{v}_2)^3 \vec{S}_1 \times \vec{v}_1 \cdot \vec{v}_2 - 64 \hat{n} \cdot \vec{v}_1 (\hat{n} \cdot \vec{v}_2)^3 \hat{n} \times \vec{S}_1 \cdot \vec{v}_2 + 32 \vec{v}_1 \cdot \vec{v}_2 (\hat{n} \cdot \vec{v}_2)^2 \hat{n} \times \vec{S}_1 \cdot \vec{v}_2 + \right.$$

$$8 \vec{v}_2 \cdot \vec{v}_2 \hat{n} \cdot \vec{v}_2 \vec{S}_1 \times \vec{v}_1 \cdot \vec{v}_2 + 32 \vec{v}_2 \cdot \vec{v}_2 \hat{n} \cdot \vec{v}_1 \hat{n} \cdot \vec{v}_2 \hat{n} \times \vec{S}_1 \cdot \vec{v}_2 - 8 \vec{v}_1 \cdot \vec{v}_2 \vec{v}_2 \cdot \vec{v}_2 \hat{n} \times \vec{S}_1 \cdot \vec{v}_2 \Big) \Big\}$$

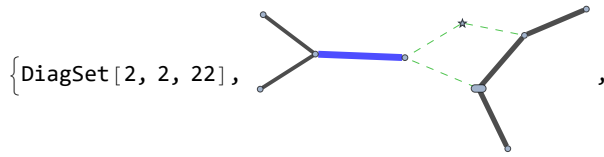

$$\begin{aligned} & \frac{1}{r} \left( - \left( \hat{n} \times \vec{S}_1 \cdot \vec{a}_1 \right) \left( \hat{n} \cdot \vec{v}_2 \right)^2 + 2 \vec{S}_1 \times \vec{a}_1 \cdot \vec{v}_2 \hat{n} \cdot \vec{v}_2 + 2 \vec{S}_1 \times \vec{a}_1 \cdot \vec{a}_2 \hat{n} \cdot \vec{v}_2 - 2 \hat{n} \times \vec{S}_1 \cdot \vec{a}_1 \hat{n} \cdot \vec{a}_2 \hat{n} \cdot \vec{v}_2 + 2 \vec{S}_1 \times \vec{a}_1 \cdot \vec{v}_2 \hat{n} \cdot \vec{a}_2 - \right. \\ & \quad \left. 2 \hat{n} \times \vec{S}_1 \cdot \vec{v}_2 \vec{a}_1 \cdot \vec{a}_2 - 2 \hat{n} \times \vec{S}_1 \cdot \vec{v}_2 \vec{a}_1 \cdot \vec{v}_2 - 2 \hat{n} \times \vec{S}_1 \cdot \vec{a}_2 \vec{a}_1 \cdot \vec{v}_2 + 2 \hat{n} \times \vec{S}_1 \cdot \vec{a}_1 \vec{v}_2 \cdot \vec{a}_2 + \hat{n} \times \vec{S}_1 \cdot \vec{a}_1 \vec{v}_2 \cdot \vec{v}_2 \right) m_1 m_2 G^2 + \\ & \frac{1}{r^2} \left( -4 \hat{n} \times \vec{S}_1 \cdot \vec{a}_1 \left( \hat{n} \cdot \vec{v}_2 \right)^3 + 5 \vec{S}_1 \times \vec{a}_1 \cdot \vec{v}_2 \left( \hat{n} \cdot \vec{v}_2 \right)^2 + \frac{4}{3} \vec{S}_1 \times \vec{v}_1 \cdot \vec{a}_1 \left( \hat{n} \cdot \vec{v}_2 \right)^2 + \frac{2}{3} \hat{n} \times \vec{S}_1 \cdot \vec{v}_1 \hat{n} \cdot \vec{v}_1 \left( \hat{n} \cdot \vec{v}_2 \right)^2 + \right. \\ & \quad \frac{10}{3} \hat{n} \times \vec{S}_1 \cdot \vec{a}_1 \hat{n} \cdot \vec{v}_1 \left( \hat{n} \cdot \vec{v}_2 \right)^2 - \frac{4}{3} \vec{S}_1 \times \vec{v}_1 \cdot \vec{v}_2 \hat{n} \cdot \vec{v}_1 \hat{n} \cdot \vec{v}_2 - \frac{8}{3} \vec{S}_1 \times \vec{a}_1 \cdot \vec{v}_2 \hat{n} \cdot \vec{v}_1 \hat{n} \cdot \vec{v}_2 - \\ & \quad \frac{4}{3} \vec{S}_1 \times \vec{v}_1 \cdot \vec{a}_2 \hat{n} \cdot \vec{v}_1 \hat{n} \cdot \vec{v}_2 + \frac{4}{3} \hat{n} \times \vec{S}_1 \cdot \vec{v}_1 \hat{n} \cdot \vec{a}_2 \hat{n} \cdot \vec{v}_1 \hat{n} \cdot \vec{v}_2 - 3 \hat{n} \times \vec{S}_1 \cdot \vec{v}_1 \vec{a}_1 \cdot \vec{v}_2 \hat{n} \cdot \vec{v}_2 - \\ & \quad 4 \hat{n} \times \vec{S}_1 \cdot \vec{v}_2 \vec{a}_1 \cdot \vec{v}_2 \hat{n} \cdot \vec{v}_2 + 3 \hat{n} \times \vec{S}_1 \cdot \vec{v}_2 \vec{v}_1 \cdot \vec{a}_1 \hat{n} \cdot \vec{v}_2 + \frac{2}{3} \hat{n} \times \vec{S}_1 \cdot \vec{v}_1 \vec{v}_1 \cdot \vec{a}_2 \hat{n} \cdot \vec{v}_2 - 3 \hat{n} \times \vec{S}_1 \cdot \vec{v}_2 \vec{v}_1 \cdot \vec{v}_1 \hat{n} \cdot \vec{v}_2 - \\ & \quad 3 \hat{n} \times \vec{S}_1 \cdot \vec{a}_2 \vec{v}_1 \cdot \vec{v}_1 \hat{n} \cdot \vec{v}_2 + \frac{2}{3} \hat{n} \times \vec{S}_1 \cdot \vec{v}_1 \vec{v}_1 \cdot \vec{v}_2 \hat{n} \cdot \vec{v}_2 + \frac{1}{3} \hat{n} \times \vec{S}_1 \cdot \vec{a}_1 \vec{v}_1 \cdot \vec{v}_2 \hat{n} \cdot \vec{v}_2 + 4 \hat{n} \times \vec{S}_1 \cdot \vec{a}_1 \vec{v}_2 \cdot \vec{v}_2 \hat{n} \cdot \vec{v}_2 - \\ & \quad \frac{4}{3} \vec{S}_1 \times \vec{v}_1 \cdot \vec{v}_2 \hat{n} \cdot \vec{a}_2 \hat{n} \cdot \vec{v}_1 + 3 \vec{S}_1 \times \vec{v}_1 \cdot \vec{v}_2 \vec{a}_1 \cdot \vec{v}_2 + 6 \hat{n} \times \vec{S}_1 \cdot \vec{v}_2 \hat{n} \cdot \vec{v}_1 \vec{a}_1 \cdot \vec{v}_2 + \frac{5}{3} \vec{S}_1 \times \vec{v}_1 \cdot \vec{v}_2 \vec{v}_1 \cdot \vec{a}_2 + \\ & \quad \hat{n} \times \vec{S}_1 \cdot \vec{v}_2 \hat{n} \cdot \vec{v}_1 \vec{v}_1 \cdot \vec{a}_2 - 3 \hat{n} \times \vec{S}_1 \cdot \vec{v}_2 \hat{n} \cdot \vec{a}_2 \vec{v}_1 \cdot \vec{v}_1 + \frac{5}{3} \vec{S}_1 \times \vec{v}_1 \cdot \vec{v}_2 \vec{v}_1 \cdot \vec{v}_2 - \frac{2}{3} \vec{S}_1 \times \vec{a}_1 \cdot \vec{v}_2 \vec{v}_1 \cdot \vec{v}_2 + \\ & \quad \frac{5}{3} \vec{S}_1 \times \vec{v}_1 \cdot \vec{a}_2 \vec{v}_1 \cdot \vec{v}_2 - 3 \hat{n} \times \vec{S}_1 \cdot \vec{v}_2 \hat{n} \cdot \vec{a}_1 \vec{v}_1 \cdot \vec{v}_2 + \frac{2}{3} \hat{n} \times \vec{S}_1 \cdot \vec{v}_1 \hat{n} \cdot \vec{a}_2 \vec{v}_1 \cdot \vec{v}_2 + \hat{n} \times \vec{S}_1 \cdot \vec{v}_2 \hat{n} \cdot \vec{v}_1 \vec{v}_1 \cdot \vec{v}_2 + \\ & \quad \hat{n} \times \vec{S}_1 \cdot \vec{a}_2 \hat{n} \cdot \vec{v}_1 \vec{v}_1 \cdot \vec{v}_2 - \frac{4}{3} \hat{n} \times \vec{S}_1 \cdot \vec{v}_1 \hat{n} \cdot \vec{v}_1 \vec{v}_2 \cdot \vec{a}_2 - 3 \vec{S}_1 \times \vec{a}_1 \cdot \vec{v}_2 \vec{v}_2 \cdot \vec{v}_2 - \frac{8}{3} \vec{S}_1 \times \vec{v}_1 \cdot \vec{a}_1 \vec{v}_2 \cdot \vec{v}_2 + \\ & \quad \left. 3 \hat{n} \times \vec{S}_1 \cdot \vec{v}_1 \hat{n} \cdot \vec{a}_1 \vec{v}_2 \cdot \vec{v}_2 - \frac{2}{3} \hat{n} \times \vec{S}_1 \cdot \vec{v}_1 \hat{n} \cdot \vec{v}_1 \vec{v}_2 \cdot \vec{v}_2 - \frac{13}{3} \hat{n} \times \vec{S}_1 \cdot \vec{a}_1 \hat{n} \cdot \vec{v}_1 \vec{v}_2 \cdot \vec{v}_2 \right) m_1 m_2 G^2 + \\ & \frac{1}{r^3} \left( -4 \hat{n} \times \vec{S}_1 \cdot \vec{v}_1 \hat{n} \cdot \vec{v}_1 \left( \hat{n} \cdot \vec{v}_2 \right)^3 - \frac{5}{2} \hat{n} \times \vec{S}_1 \cdot \vec{v}_1 \left( \hat{n} \cdot \vec{v}_1 \right)^2 \left( \hat{n} \cdot \vec{v}_2 \right)^2 - 6 \vec{S}_1 \times \vec{v}_1 \cdot \vec{v}_2 \hat{n} \cdot \vec{v}_1 \left( \hat{n} \cdot \vec{v}_2 \right)^2 - \right. \\ & \quad \frac{5}{6} \hat{n} \times \vec{S}_1 \cdot \vec{v}_1 \vec{v}_1 \cdot \vec{v}_1 \left( \hat{n} \cdot \vec{v}_2 \right)^2 - 12 \hat{n} \times \vec{S}_1 \cdot \vec{v}_2 \vec{v}_1 \cdot \vec{v}_1 \left( \hat{n} \cdot \vec{v}_2 \right)^2 + 2 \hat{n} \times \vec{S}_1 \cdot \vec{v}_1 \vec{v}_1 \cdot \vec{v}_2 \left( \hat{n} \cdot \vec{v}_2 \right)^2 + \\ & \quad \frac{7}{3} \vec{S}_1 \times \vec{v}_1 \cdot \vec{v}_2 \left( \hat{n} \cdot \vec{v}_1 \right)^2 \hat{n} \cdot \vec{v}_2 + \frac{2}{3} \vec{S}_1 \times \vec{v}_1 \cdot \vec{v}_2 \vec{v}_1 \cdot \vec{v}_1 \hat{n} \cdot \vec{v}_2 + 8 \hat{n} \times \vec{S}_1 \cdot \vec{v}_2 \hat{n} \cdot \vec{v}_1 \vec{v}_1 \cdot \vec{v}_1 \hat{n} \cdot \vec{v}_2 + \\ & \quad 4 \vec{S}_1 \times \vec{v}_1 \cdot \vec{v}_2 \vec{v}_1 \cdot \vec{v}_2 \hat{n} \cdot \vec{v}_2 + \frac{2}{3} \hat{n} \times \vec{S}_1 \cdot \vec{v}_1 \hat{n} \cdot \vec{v}_1 \vec{v}_1 \cdot \vec{v}_2 \hat{n} \cdot \vec{v}_2 + 4 \hat{n} \times \vec{S}_1 \cdot \vec{v}_2 \hat{n} \cdot \vec{v}_1 \vec{v}_1 \cdot \vec{v}_2 \hat{n} \cdot \vec{v}_2 - \\ & \quad 4 \hat{n} \times \vec{S}_1 \cdot \vec{v}_1 \hat{n} \cdot \vec{v}_1 \vec{v}_2 \cdot \vec{v}_2 \hat{n} \cdot \vec{v}_2 - \frac{1}{3} \hat{n} \times \vec{S}_1 \cdot \vec{v}_1 \left( \vec{v}_1 \cdot \vec{v}_2 \right)^2 - \hat{n} \times \vec{S}_1 \cdot \vec{v}_2 \left( \vec{v}_1 \cdot \vec{v}_2 \right)^2 - \\ & \quad 2 \hat{n} \times \vec{S}_1 \cdot \vec{v}_2 \left( \hat{n} \cdot \vec{v}_1 \right)^2 \vec{v}_1 \cdot \vec{v}_2 - \frac{5}{3} \vec{S}_1 \times \vec{v}_1 \cdot \vec{v}_2 \hat{n} \cdot \vec{v}_1 \vec{v}_1 \cdot \vec{v}_2 + \frac{7}{6} \hat{n} \times \vec{S}_1 \cdot \vec{v}_1 \left( \hat{n} \cdot \vec{v}_1 \right)^2 \vec{v}_2 \cdot \vec{v}_2 + \\ & \quad \left. 2 \vec{S}_1 \times \vec{v}_1 \cdot \vec{v}_2 \hat{n} \cdot \vec{v}_1 \vec{v}_2 \cdot \vec{v}_2 - \frac{1}{6} \hat{n} \times \vec{S}_1 \cdot \vec{v}_1 \vec{v}_1 \cdot \vec{v}_1 \vec{v}_2 \cdot \vec{v}_2 + 3 \hat{n} \times \vec{S}_1 \cdot \vec{v}_2 \vec{v}_1 \cdot \vec{v}_1 \vec{v}_2 \cdot \vec{v}_2 \right) m_1 m_2 G^2 \Big\} \end{aligned}$$

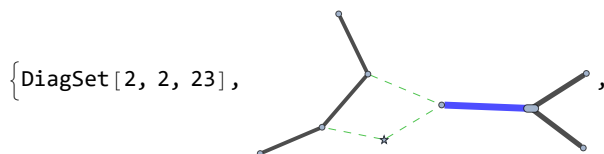

$$\frac{1}{r} G^2 \left( -4 \hat{n} \times \vec{S}_1 \cdot \vec{v}_2 \vec{a}_1 \cdot \vec{a}_2 + 4 \hat{n} \times \vec{a}_2 \cdot \vec{S}_1 \vec{a}_1 \cdot \vec{v}_2 + 4 \hat{n} \times \vec{S}_1 \cdot \vec{v}_1 \vec{a}_2 \cdot \vec{a}_2 - 4 \hat{n} \times \vec{S}_1 \cdot \vec{v}_2 \vec{a}_2 \cdot \vec{v}_1 + \right.$$

$$\begin{aligned}
& 8 \hat{n} \times \vec{a}_2 \cdot \vec{S}_1 \vec{a}_2 \cdot \vec{v}_1 + 4 \hat{n} \times \vec{S}_1 \cdot \vec{v}_1 \vec{a}_2 \cdot \vec{v}_2 - 4 \hat{n} \times \vec{a}_1 \cdot \vec{S}_1 \vec{a}_2 \cdot \vec{v}_2 + 4 \hat{n} \times \vec{a}_2 \cdot \vec{S}_1 \vec{v}_1 \cdot \vec{v}_2 \Big) m_2^2 + \frac{1}{r^2} \\
& G^2 \Big( 4 \vec{S}_1 \times \vec{v}_1 \cdot \vec{v}_2 \vec{a}_2 \cdot \vec{v}_1 + 8 \hat{n} \times \vec{S}_1 \cdot \vec{v}_2 \hat{n} \cdot \vec{v}_1 \vec{a}_2 \cdot \vec{v}_1 - 16 \hat{n} \times \vec{S}_1 \cdot \vec{v}_2 \hat{n} \cdot \vec{v}_2 \vec{a}_2 \cdot \vec{v}_1 - 16 \vec{S}_1 \times \vec{v}_1 \cdot \vec{v}_2 \vec{a}_2 \cdot \vec{v}_2 - \\
& 8 \hat{n} \times \vec{S}_1 \cdot \vec{v}_1 \hat{n} \cdot \vec{v}_1 \vec{a}_2 \cdot \vec{v}_2 - 8 \hat{n} \times \vec{S}_1 \cdot \vec{v}_2 \hat{n} \cdot \vec{v}_1 \vec{a}_2 \cdot \vec{v}_2 + 24 \hat{n} \times \vec{S}_1 \cdot \vec{v}_1 \hat{n} \cdot \vec{v}_2 \vec{a}_2 \cdot \vec{v}_2 + 4 \vec{a}_2 \times \vec{S}_1 \cdot \vec{v}_1 \vec{v}_1 \cdot \vec{v}_2 - 16 \vec{a}_2 \times \vec{S}_1 \cdot \vec{v}_1 \vec{v}_2 \cdot \vec{v}_2 - \\
& \vec{v}_1 \cdot \vec{v}_2 + 16 \hat{n} \times \vec{S}_1 \cdot \vec{v}_2 \hat{n} \cdot \vec{a}_2 \vec{v}_1 \cdot \vec{v}_2 - 8 \hat{n} \times \vec{a}_2 \cdot \vec{S}_1 \hat{n} \cdot \vec{v}_1 \vec{v}_1 \cdot \vec{v}_2 + 16 \hat{n} \times \vec{a}_2 \cdot \vec{S}_1 \hat{n} \cdot \vec{v}_2 \vec{v}_1 \cdot \vec{v}_2 + 2 \vec{S}_1 \times \vec{v}_1 \cdot \vec{v}_2 \vec{v}_2 \cdot \vec{v}_2 - \\
& 2 \vec{a}_1 \times \vec{S}_1 \cdot \vec{v}_2 \vec{v}_2 \cdot \vec{v}_2 + 12 \vec{a}_2 \times \vec{S}_1 \cdot \vec{v}_1 \vec{v}_2 \cdot \vec{v}_2 + 2 \hat{n} \times \vec{S}_1 \cdot \vec{v}_2 \hat{n} \cdot \vec{a}_1 \vec{v}_2 \cdot \vec{v}_2 - 16 \hat{n} \times \vec{S}_1 \cdot \vec{v}_1 \hat{n} \cdot \vec{a}_2 \vec{v}_2 \cdot \vec{v}_2 + \\
& 2 \hat{n} \times \vec{S}_1 \cdot \vec{v}_2 \hat{n} \cdot \vec{v}_1 \vec{v}_2 \cdot \vec{v}_2 - 8 \hat{n} \times \vec{a}_2 \cdot \vec{S}_1 \hat{n} \cdot \vec{v}_1 \vec{v}_2 \cdot \vec{v}_2 - 2 \hat{n} \times \vec{S}_1 \cdot \vec{v}_1 \hat{n} \cdot \vec{v}_2 \vec{v}_2 \cdot \vec{v}_2 + 2 \hat{n} \times \vec{a}_1 \cdot \vec{S}_1 \hat{n} \cdot \vec{v}_2 \vec{v}_2 \cdot \vec{v}_2 \Big) m_2^2 + \\
& \frac{1}{r^3} G^2 \Big( -8 \hat{n} \times \vec{S}_1 \cdot \vec{v}_2 \vec{v}_2 \cdot \vec{v}_2 (\hat{n} \cdot \vec{v}_1)^2 - 6 \vec{S}_1 \times \vec{v}_1 \cdot \vec{v}_2 \vec{v}_2 \cdot \vec{v}_2 \hat{n} \cdot \vec{v}_1 + 8 \hat{n} \times \vec{S}_1 \cdot \vec{v}_1 \hat{n} \cdot \vec{v}_2 \vec{v}_2 \cdot \vec{v}_2 \hat{n} \cdot \vec{v}_1 + 8 \hat{n} \times \vec{S}_1 \cdot \vec{v}_2 \\
& \hat{n} \cdot \vec{v}_2 \vec{v}_2 \cdot \vec{v}_2 \hat{n} \cdot \vec{v}_1 - 2 \hat{n} \times \vec{S}_1 \cdot \vec{v}_1 (\vec{v}_2 \cdot \vec{v}_2)^2 + 8 \hat{n} \times \vec{S}_1 \cdot \vec{v}_2 (\hat{n} \cdot \vec{v}_2)^2 \vec{v}_1 \cdot \vec{v}_2 - 12 \hat{n} \times \vec{S}_1 \cdot \vec{v}_1 (\hat{n} \cdot \vec{v}_2)^2 \vec{v}_2 \cdot \vec{v}_2 + \\
& 8 \vec{S}_1 \times \vec{v}_1 \cdot \vec{v}_2 \hat{n} \cdot \vec{v}_2 \vec{v}_2 \cdot \vec{v}_2 + 2 \hat{n} \times \vec{S}_1 \cdot \vec{v}_2 \vec{v}_1 \cdot \vec{v}_1 \vec{v}_2 \cdot \vec{v}_2 - 2 \hat{n} \times \vec{S}_1 \cdot \vec{v}_1 \vec{v}_1 \cdot \vec{v}_2 \vec{v}_2 \cdot \vec{v}_2 + 4 \hat{n} \times \vec{S}_1 \cdot \vec{v}_2 \vec{v}_1 \cdot \vec{v}_2 \vec{v}_2 \cdot \vec{v}_2 \Big) m_2^2 \Big\}
\end{aligned}$$

$\{\text{DiagSet}[2, 2, 24],$

$$\begin{aligned} & \frac{1}{r} \left( 6 \vec{S}_1 \times \vec{v}_1 \cdot \vec{v}_2 \hat{n} \cdot \vec{a}_1 + 2 \vec{S}_1 \times \vec{a}_1 \cdot \vec{v}_2 \hat{n} \cdot \vec{a}_1 + 6 \vec{S}_1 \times \vec{v}_1 \cdot \vec{a}_2 \hat{n} \cdot \vec{a}_1 - 6 \vec{S}_1 \times \vec{v}_1 \cdot \vec{a}_1 \hat{n} \cdot \vec{a}_2 - 4 \vec{S}_1 \times \vec{a}_1 \cdot \vec{v}_2 \hat{n} \cdot \vec{v}_1 - \right. \\ & 4 \vec{S}_1 \times \vec{a}_1 \cdot \vec{a}_2 \hat{n} \cdot \vec{v}_1 - 6 \vec{S}_1 \times \vec{v}_1 \cdot \vec{a}_1 \hat{n} \cdot \vec{v}_2 + 2 \hat{n} \times \vec{S}_1 \cdot \vec{v}_2 \vec{a}_1 \cdot \vec{a}_1 - 2 \hat{n} \times \vec{S}_1 \cdot \vec{v}_1 \vec{a}_1 \cdot \vec{a}_2 - 2 \hat{n} \times \vec{S}_1 \cdot \vec{v}_1 \vec{a}_1 \cdot \vec{v}_2 - \\ & 4 \hat{n} \times \vec{S}_1 \cdot \vec{a}_1 \vec{a}_1 \cdot \vec{v}_2 + 2 \hat{n} \times \vec{S}_1 \cdot \vec{v}_2 \vec{v}_1 \cdot \vec{a}_1 + 2 \hat{n} \times \vec{S}_1 \cdot \vec{a}_2 \vec{v}_1 \cdot \vec{a}_1 - 2 \hat{n} \times \vec{S}_1 \cdot \vec{a}_1 \vec{v}_1 \cdot \vec{a}_2 - 2 \hat{n} \times \vec{S}_1 \cdot \vec{a}_1 \vec{v}_1 \cdot \vec{v}_2 \left. \right) m_1 m_2 G^2 + \\ & \frac{1}{r^3} \left( 2 \vec{S}_1 \times \vec{v}_1 \cdot \vec{v}_2 (\hat{n} \cdot \vec{v}_1)^3 - 4 \vec{S}_1 \times \vec{v}_1 \cdot \vec{v}_2 \hat{n} \cdot \vec{v}_2 (\hat{n} \cdot \vec{v}_1)^2 - 6 \hat{n} \times \vec{S}_1 \cdot \vec{v}_2 \vec{v}_1 \cdot \vec{v}_1 (\hat{n} \cdot \vec{v}_1)^2 - \right. \\ & 4 \hat{n} \times \vec{S}_1 \cdot \vec{v}_1 \vec{v}_1 \cdot \vec{v}_2 (\hat{n} \cdot \vec{v}_1)^2 - 4 \vec{S}_1 \times \vec{v}_1 \cdot \vec{v}_2 \vec{v}_1 \cdot \vec{v}_1 \hat{n} \cdot \vec{v}_1 + 8 \hat{n} \times \vec{S}_1 \cdot \vec{v}_2 \hat{n} \cdot \vec{v}_2 \vec{v}_1 \cdot \vec{v}_1 \hat{n} \cdot \vec{v}_1 - \\ & 2 \vec{S}_1 \times \vec{v}_1 \cdot \vec{v}_2 \vec{v}_1 \cdot \vec{v}_2 \hat{n} \cdot \vec{v}_1 + 16 \hat{n} \times \vec{S}_1 \cdot \vec{v}_1 \hat{n} \cdot \vec{v}_2 \vec{v}_1 \cdot \vec{v}_2 \hat{n} \cdot \vec{v}_1 - 4 \hat{n} \times \vec{S}_1 \cdot \vec{v}_1 (\vec{v}_1 \cdot \vec{v}_2)^2 + \\ & 2 \vec{S}_1 \times \vec{v}_1 \cdot \vec{v}_2 \hat{n} \cdot \vec{v}_2 \vec{v}_1 \cdot \vec{v}_1 + 4 \hat{n} \times \vec{S}_1 \cdot \vec{v}_1 \vec{v}_1 \cdot \vec{v}_1 \vec{v}_1 \cdot \vec{v}_2 - 2 \hat{n} \times \vec{S}_1 \cdot \vec{v}_2 \vec{v}_1 \cdot \vec{v}_1 \vec{v}_1 \cdot \vec{v}_2 \left. \right) m_1 m_2 G^2 + \frac{1}{r^2} \\ & \left( - \left( \vec{S}_1 \times \vec{v}_1 \cdot \vec{v}_2 \right) (\hat{n} \cdot \vec{v}_1)^2 + 3 \vec{S}_1 \times \vec{a}_1 \cdot \vec{v}_2 (\hat{n} \cdot \vec{v}_1)^2 - \vec{S}_1 \times \vec{v}_1 \cdot \vec{a}_2 (\hat{n} \cdot \vec{v}_1)^2 - 7 \vec{S}_1 \times \vec{v}_1 \cdot \vec{v}_2 \hat{n} \cdot \vec{a}_1 \hat{n} \cdot \vec{v}_1 - \right. \\ & 8 \vec{S}_1 \times \vec{a}_1 \cdot \vec{v}_2 \hat{n} \cdot \vec{v}_2 \hat{n} \cdot \vec{v}_1 + 6 \vec{S}_1 \times \vec{v}_1 \cdot \vec{a}_1 \hat{n} \cdot \vec{v}_2 \hat{n} \cdot \vec{v}_1 + 5 \hat{n} \times \vec{S}_1 \cdot \vec{v}_1 \vec{a}_1 \cdot \vec{v}_2 \hat{n} \cdot \vec{v}_1 - \\ & 10 \hat{n} \times \vec{S}_1 \cdot \vec{v}_2 \vec{v}_1 \cdot \vec{a}_1 \hat{n} \cdot \vec{v}_1 + 4 \hat{n} \times \vec{S}_1 \cdot \vec{v}_1 \vec{v}_1 \cdot \vec{a}_2 \hat{n} \cdot \vec{v}_1 + 2 \hat{n} \times \vec{S}_1 \cdot \vec{v}_2 \vec{v}_1 \cdot \vec{v}_1 \hat{n} \cdot \vec{v}_1 + \\ & 2 \hat{n} \times \vec{S}_1 \cdot \vec{a}_2 \vec{v}_1 \cdot \vec{v}_1 \hat{n} \cdot \vec{v}_1 + 4 \hat{n} \times \vec{S}_1 \cdot \vec{v}_1 \vec{v}_1 \cdot \vec{v}_2 \hat{n} \cdot \vec{v}_1 + 4 \hat{n} \times \vec{S}_1 \cdot \vec{a}_1 \vec{v}_1 \cdot \vec{v}_2 \hat{n} \cdot \vec{v}_1 - 12 \vec{S}_1 \times \vec{v}_1 \cdot \vec{a}_1 (\hat{n} \cdot \vec{v}_2)^2 + \\ & 12 \vec{S}_1 \times \vec{v}_1 \cdot \vec{v}_2 \hat{n} \cdot \vec{a}_1 \hat{n} \cdot \vec{v}_2 - 4 \vec{S}_1 \times \vec{v}_1 \cdot \vec{v}_2 \vec{a}_1 \cdot \vec{v}_2 - 4 \hat{n} \times \vec{S}_1 \cdot \vec{v}_1 \hat{n} \cdot \vec{v}_2 \vec{a}_1 \cdot \vec{v}_2 - 6 \vec{S}_1 \times \vec{v}_1 \cdot \vec{v}_2 \vec{v}_1 \cdot \vec{a}_1 + \\ & 9 \hat{n} \times \vec{S}_1 \cdot \vec{v}_1 \hat{n} \cdot \vec{v}_2 \vec{v}_1 \cdot \vec{a}_1 + 4 \hat{n} \times \vec{S}_1 \cdot \vec{v}_2 \hat{n} \cdot \vec{v}_2 \vec{v}_1 \cdot \vec{a}_1 + \vec{S}_1 \times \vec{v}_1 \cdot \vec{v}_2 \vec{v}_1 \cdot \vec{v}_1 + 6 \vec{S}_1 \times \vec{a}_1 \cdot \vec{v}_2 \vec{v}_1 \cdot \vec{v}_1 + \\ & \vec{S}_1 \times \vec{v}_1 \cdot \vec{a}_2 \vec{v}_1 \cdot \vec{v}_1 + 6 \hat{n} \times \vec{S}_1 \cdot \vec{v}_2 \hat{n} \cdot \vec{a}_1 \vec{v}_1 \cdot \vec{v}_1 - 9 \hat{n} \times \vec{S}_1 \cdot \vec{a}_1 \hat{n} \cdot \vec{v}_2 \vec{v}_1 \cdot \vec{v}_1 + 6 \vec{S}_1 \times \vec{a}_1 \cdot \vec{v}_2 \vec{v}_1 \cdot \vec{v}_2 + \\ & \left. \vec{S}_1 \times \vec{v}_1 \cdot \vec{a}_1 \vec{v}_1 \cdot \vec{v}_2 - \hat{n} \times \vec{S}_1 \cdot \vec{v}_1 \hat{n} \cdot \vec{a}_1 \vec{v}_1 \cdot \vec{v}_2 - 4 \hat{n} \times \vec{S}_1 \cdot \vec{a}_1 \hat{n} \cdot \vec{v}_2 \vec{v}_1 \cdot \vec{v}_2 + 6 \vec{S}_1 \times \vec{v}_1 \cdot \vec{a}_1 \vec{v}_2 \cdot \vec{v}_2 \right) m_1 m_2 G^2 \} \end{aligned}$$

$\{\text{DiagSet}[2, 2, 25],$

$$\frac{1}{r} \left( 2 \hat{n} \times \vec{S_1} \cdot \vec{a_2} (\hat{n} \cdot \vec{v_1})^2 + 4 \hat{n} \times \vec{S_1} \cdot \vec{a_2} \hat{n} \cdot \vec{a_1} \hat{n} \cdot \vec{v_1} - \hat{n} \times \vec{S_1} \cdot \vec{v_1} \vec{a_1} \cdot \vec{a_2} - \hat{n} \times \vec{S_1} \cdot \vec{v_1} \vec{v_1} \cdot \vec{a_2} - \hat{n} \times \vec{S_1} \cdot \vec{a_1} \vec{v_1} \cdot \vec{a_2} \right) m_1 m_2 G^2 +$$

$$\begin{aligned} & \frac{1}{r^2} \left( -8 \hat{n} \times \vec{S}_1 \cdot \vec{a}_2 (\hat{n} \cdot \vec{v}_1)^3 - 2 \vec{S}_1 \times \vec{v}_1 \cdot \vec{a}_2 (\hat{n} \cdot \vec{v}_1)^2 + 8 \hat{n} \times \vec{S}_1 \cdot \vec{v}_2 \hat{n} \cdot \vec{v}_2 (\hat{n} \cdot \vec{v}_1)^2 + 16 \hat{n} \times \vec{S}_1 \cdot \vec{v}_2 \hat{n} \cdot \vec{a}_1 \hat{n} \cdot \vec{v}_2 \hat{n} \cdot \vec{v}_1 - \right. \\ & 4 \hat{n} \times \vec{S}_1 \cdot \vec{v}_2 \vec{a}_1 \cdot \vec{v}_2 \hat{n} \cdot \vec{v}_1 + 2 \hat{n} \times \vec{S}_1 \cdot \vec{v}_1 \vec{v}_1 \cdot \vec{a}_2 \hat{n} \cdot \vec{v}_1 + 4 \hat{n} \times \vec{S}_1 \cdot \vec{a}_2 \vec{v}_1 \cdot \vec{v}_1 \hat{n} \cdot \vec{v}_1 - 4 \hat{n} \times \vec{S}_1 \cdot \vec{v}_2 \vec{v}_1 \cdot \vec{v}_2 \hat{n} \cdot \vec{v}_1 + \\ & \vec{S}_1 \times \vec{v}_1 \cdot \vec{v}_2 \vec{a}_1 \cdot \vec{v}_2 - 2 \hat{n} \times \vec{S}_1 \cdot \vec{v}_1 \hat{n} \cdot \vec{v}_2 \vec{a}_1 \cdot \vec{v}_2 + \vec{S}_1 \times \vec{v}_1 \cdot \vec{v}_2 \vec{v}_1 \cdot \vec{v}_2 + \vec{S}_1 \times \vec{a}_1 \cdot \vec{v}_2 \vec{v}_1 \cdot \vec{v}_2 - \\ & \left. 4 \hat{n} \times \vec{S}_1 \cdot \vec{v}_2 \hat{n} \cdot \vec{a}_1 \vec{v}_1 \cdot \vec{v}_2 - 2 \hat{n} \times \vec{S}_1 \cdot \vec{v}_1 \hat{n} \cdot \vec{v}_2 \vec{v}_1 \cdot \vec{v}_2 - 2 \hat{n} \times \vec{S}_1 \cdot \vec{a}_1 \hat{n} \cdot \vec{v}_2 \vec{v}_1 \cdot \vec{v}_2 \right) m_1 m_2 G^2 + \\ & \frac{1}{r^3} \left( -48 \hat{n} \times \vec{S}_1 \cdot \vec{v}_2 \hat{n} \cdot \vec{v}_2 (\hat{n} \cdot \vec{v}_1)^3 - 8 \vec{S}_1 \times \vec{v}_1 \cdot \vec{v}_2 \hat{n} \cdot \vec{v}_2 (\hat{n} \cdot \vec{v}_1)^2 + 24 \hat{n} \times \vec{S}_1 \cdot \vec{v}_2 \vec{v}_1 \cdot \vec{v}_2 (\hat{n} \cdot \vec{v}_1)^2 + \right. \\ & 16 \hat{n} \times \vec{S}_1 \cdot \vec{v}_2 \hat{n} \cdot \vec{v}_2 \vec{v}_1 \cdot \vec{v}_1 \hat{n} \cdot \vec{v}_1 + 2 \vec{S}_1 \times \vec{v}_1 \cdot \vec{v}_2 \vec{v}_1 \cdot \vec{v}_2 \hat{n} \cdot \vec{v}_1 + \\ & \left. 8 \hat{n} \times \vec{S}_1 \cdot \vec{v}_1 \hat{n} \cdot \vec{v}_2 \vec{v}_1 \cdot \vec{v}_2 \hat{n} \cdot \vec{v}_1 - 2 \hat{n} \times \vec{S}_1 \cdot \vec{v}_1 (\vec{v}_1 \cdot \vec{v}_2)^2 - 4 \hat{n} \times \vec{S}_1 \cdot \vec{v}_2 \vec{v}_1 \cdot \vec{v}_1 \vec{v}_1 \cdot \vec{v}_2 \right) m_1 m_2 G^2 \} \end{aligned}$$

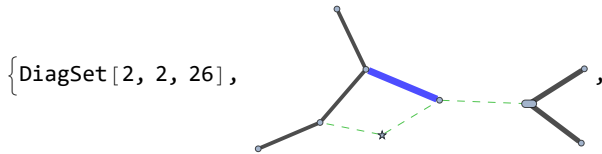

$$\begin{aligned} & \frac{1}{r} G^2 \left( -\frac{8}{3} \hat{n} \times \vec{a}_2 \cdot \vec{S}_1 (\hat{n} \cdot \vec{v}_2)^2 + \frac{8}{3} \vec{a}_2 \times \vec{S}_1 \cdot \vec{v}_2 \hat{n} \cdot \vec{v}_2 - \frac{16}{3} \hat{n} \times \vec{a}_2 \cdot \vec{S}_1 \hat{n} \cdot \vec{a}_2 \hat{n} \cdot \vec{v}_2 + \frac{8}{3} \vec{a}_2 \times \vec{S}_1 \cdot \vec{v}_2 \hat{n} \cdot \vec{a}_2 - \right. \\ & 4 \hat{n} \times \vec{S}_1 \cdot \vec{v}_2 \vec{a}_2 \cdot \vec{a}_2 - 4 \hat{n} \times \vec{S}_1 \cdot \vec{v}_2 \vec{a}_2 \cdot \vec{v}_2 - \frac{4}{3} \hat{n} \times \vec{a}_2 \cdot \vec{S}_1 \vec{a}_2 \cdot \vec{v}_2 - \frac{8}{3} \hat{n} \times \vec{a}_2 \cdot \vec{S}_1 \vec{v}_2 \cdot \vec{v}_2 \left. \right) m_2^2 + \frac{1}{r^2} \\ & G^2 \left( \frac{16}{3} \hat{n} \times \vec{S}_1 \cdot \vec{v}_2 (\hat{n} \cdot \vec{v}_2)^3 - \frac{16}{3} \hat{n} \times \vec{a}_2 \cdot \vec{S}_1 (\hat{n} \cdot \vec{v}_2)^3 - \frac{8}{3} \vec{a}_2 \times \vec{S}_1 \cdot \vec{v}_1 (\hat{n} \cdot \vec{v}_2)^2 + \frac{4}{3} \vec{a}_2 \times \vec{S}_1 \cdot \vec{v}_2 (\hat{n} \cdot \vec{v}_2)^2 + \right. \\ & \frac{32}{3} \hat{n} \times \vec{S}_1 \cdot \vec{v}_2 \hat{n} \cdot \vec{a}_2 (\hat{n} \cdot \vec{v}_2)^2 + \frac{32}{3} \hat{n} \times \vec{a}_2 \cdot \vec{S}_1 \hat{n} \cdot \vec{v}_1 (\hat{n} \cdot \vec{v}_2)^2 - \frac{16}{3} \vec{a}_2 \times \vec{S}_1 \cdot \vec{v}_2 \hat{n} \cdot \vec{v}_1 \hat{n} \cdot \vec{v}_2 - \\ & \frac{4}{3} \hat{n} \times \vec{S}_1 \cdot \vec{v}_2 \vec{a}_2 \cdot \vec{v}_2 \hat{n} \cdot \vec{v}_2 - \frac{16}{3} \hat{n} \times \vec{a}_2 \cdot \vec{S}_1 \vec{v}_1 \cdot \vec{v}_2 \hat{n} \cdot \vec{v}_2 - 8 \hat{n} \times \vec{S}_1 \cdot \vec{v}_2 \vec{v}_2 \cdot \vec{v}_2 \hat{n} \cdot \vec{v}_2 + \\ & 8 \hat{n} \times \vec{a}_2 \cdot \vec{S}_1 \vec{v}_2 \cdot \vec{v}_2 \hat{n} \cdot \vec{v}_2 + 4 \vec{S}_1 \times \vec{v}_1 \cdot \vec{v}_2 \vec{a}_2 \cdot \vec{v}_2 + 8 \hat{n} \times \vec{S}_1 \cdot \vec{v}_2 \hat{n} \cdot \vec{v}_1 \vec{a}_2 \cdot \vec{v}_2 + \frac{8}{3} \vec{a}_2 \times \vec{S}_1 \cdot \vec{v}_2 \vec{v}_1 \cdot \vec{v}_2 - \\ & \frac{8}{3} \vec{a}_2 \times \vec{S}_1 \cdot \vec{v}_1 \vec{v}_2 \cdot \vec{v}_2 - \frac{2}{3} \vec{a}_2 \times \vec{S}_1 \cdot \vec{v}_2 \vec{v}_2 \cdot \vec{v}_2 - \frac{20}{3} \hat{n} \times \vec{S}_1 \cdot \vec{v}_2 \hat{n} \cdot \vec{a}_2 \vec{v}_2 \cdot \vec{v}_2 + \frac{16}{3} \hat{n} \times \vec{a}_2 \cdot \vec{S}_1 \hat{n} \cdot \vec{v}_1 \vec{v}_2 \cdot \vec{v}_2 \left. \right) m_2^2 + \\ & \frac{1}{r^3} G^2 \left( 8 \hat{n} \times \vec{S}_1 \cdot \vec{v}_2 (\hat{n} \cdot \vec{v}_2)^4 - \frac{16}{3} \vec{S}_1 \times \vec{v}_1 \cdot \vec{v}_2 (\hat{n} \cdot \vec{v}_2)^3 - 32 \hat{n} \times \vec{S}_1 \cdot \vec{v}_2 \hat{n} \cdot \vec{v}_1 (\hat{n} \cdot \vec{v}_2)^3 + \right. \\ & 16 \hat{n} \times \vec{S}_1 \cdot \vec{v}_2 \vec{v}_1 \cdot \vec{v}_2 (\hat{n} \cdot \vec{v}_2)^2 - 12 \hat{n} \times \vec{S}_1 \cdot \vec{v}_2 \vec{v}_2 \cdot \vec{v}_2 (\hat{n} \cdot \vec{v}_2)^2 + 8 \vec{S}_1 \times \vec{v}_1 \cdot \vec{v}_2 \vec{v}_2 \cdot \vec{v}_2 \hat{n} \cdot \vec{v}_2 + \\ & \left. 32 \hat{n} \times \vec{S}_1 \cdot \vec{v}_2 \hat{n} \cdot \vec{v}_1 \vec{v}_2 \cdot \vec{v}_2 \hat{n} \cdot \vec{v}_2 + 2 \hat{n} \times \vec{S}_1 \cdot \vec{v}_2 (\vec{v}_2 \cdot \vec{v}_2)^2 - 8 \hat{n} \times \vec{S}_1 \cdot \vec{v}_2 \vec{v}_1 \cdot \vec{v}_2 \vec{v}_2 \cdot \vec{v}_2 \right) m_2^2 \} \end{aligned}$$

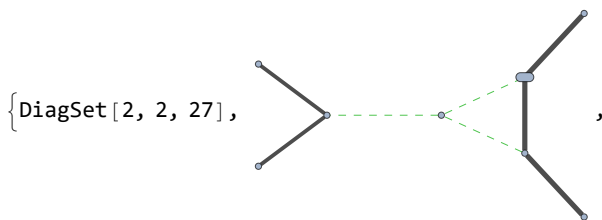

$$\begin{aligned} & \frac{1}{r} \left( -32 \vec{S}_1 \times \vec{a}_1 \cdot \vec{v}_2 \hat{n} \cdot \vec{v}_1 + 8 \vec{S}_1 \times \vec{v}_1 \cdot \vec{a}_2 \hat{n} \cdot \vec{v}_1 - 16 \vec{S}_1 \times \vec{v}_1 \cdot \vec{v}_2 \hat{n} \cdot \vec{v}_1 - \right. \\ & 16 \vec{S}_1 \times \vec{a}_1 \cdot \vec{v}_2 \hat{n} \cdot \vec{v}_1 + 8 \vec{S}_1 \times \vec{a}_1 \cdot \vec{a}_2 \hat{n} \cdot \vec{v}_1 - 8 \vec{S}_1 \times \vec{v}_1 \cdot \vec{a}_1 \hat{n} \cdot \vec{v}_2 - 8 \vec{S}_1 \times \vec{v}_1 \cdot \vec{a}_1 \hat{n} \cdot \vec{v}_2 - \\ & \left. 16 \hat{n} \times \vec{S}_1 \cdot \vec{v}_1 \vec{a}_1 \cdot \vec{v}_2 - 16 \hat{n} \times \vec{S}_1 \cdot \vec{a}_1 \vec{a}_1 \cdot \vec{v}_2 + 8 \hat{n} \times \vec{S}_1 \cdot \vec{v}_1 \vec{v}_1 \cdot \vec{a}_2 + 8 \hat{n} \times \vec{S}_1 \cdot \vec{a}_1 \vec{v}_1 \cdot \vec{a}_2 \right) m_1 m_2 G^2 + \frac{1}{r^2} \\ & \left( 20 \vec{S}_1 \times \vec{v}_1 \cdot \vec{v}_2 (\hat{n} \cdot \vec{v}_1)^2 + 20 \vec{S}_1 \times \vec{a}_1 \cdot \vec{v}_2 (\hat{n} \cdot \vec{v}_1)^2 - 3 \vec{S}_1 \times \vec{v}_1 \cdot \vec{a}_2 (\hat{n} \cdot \vec{v}_1)^2 + 4 \vec{S}_1 \times \vec{v}_1 \cdot \vec{v}_2 \hat{n} \cdot \vec{a}_1 \hat{n} \cdot \vec{v}_1 + \right. \end{aligned}$$

$$\begin{aligned} & 16 \vec{S_1} \times \vec{v_1} \cdot \vec{v_2} \hat{n} \cdot \vec{v_2} \hat{n} \cdot \vec{v_1} + 16 \vec{S_1} \times \vec{v_1} \cdot \vec{v_2} \hat{n} \cdot \vec{v_2} \hat{n} \cdot \vec{v_1} + 6 \vec{S_1} \times \vec{v_1} \cdot \vec{a_1} \hat{n} \cdot \vec{v_2} \hat{n} \cdot \vec{v_1} + 28 \hat{n} \times \vec{S_1} \cdot \vec{v_1} \vec{a_1} \cdot \vec{v_2} \hat{n} \cdot \vec{v_1} - \\ & 13 \hat{n} \times \vec{S_1} \cdot \vec{v_1} \vec{v_1} \cdot \vec{a_2} \hat{n} \cdot \vec{v_1} + 4 \hat{n} \times \vec{S_1} \cdot \vec{v_2} \vec{v_1} \cdot \vec{v_1} \hat{n} \cdot \vec{v_1} - 3 \hat{n} \times \vec{S_1} \cdot \vec{a_2} \vec{v_1} \cdot \vec{v_1} \hat{n} \cdot \vec{v_1} + 28 \hat{n} \times \vec{S_1} \cdot \vec{v_1} \vec{v_1} \cdot \vec{v_2} \hat{n} \cdot \vec{v_1} + \\ & 28 \hat{n} \times \vec{S_1} \cdot \vec{a_1} \vec{v_1} \cdot \vec{v_2} \hat{n} \cdot \vec{v_1} - 6 \hat{n} \times \vec{S_1} \cdot \vec{v_2} \vec{v_2} \cdot \vec{a_2} \hat{n} \cdot \vec{v_1} + 4 \hat{n} \times \vec{S_1} \cdot \vec{v_2} \vec{v_2} \cdot \vec{v_2} \hat{n} \cdot \vec{v_1} - 3 \hat{n} \times \vec{S_1} \cdot \vec{a_2} \vec{v_2} \cdot \vec{v_2} \hat{n} \cdot \vec{v_1} + \\ & 6 \vec{S_1} \times \vec{v_1} \cdot \vec{v_2} \vec{v_1} \cdot \vec{a_1} - 18 \hat{n} \times \vec{S_1} \cdot \vec{v_1} \hat{n} \cdot \vec{v_2} \vec{v_1} \cdot \vec{a_1} - 4 \vec{S_1} \times \vec{v_1} \cdot \vec{v_2} \vec{v_1} \cdot \vec{v_1} - 6 \vec{S_1} \times \vec{a_1} \cdot \vec{v_2} \vec{v_1} \cdot \vec{v_1} - \\ & 4 \hat{n} \times \vec{S_1} \cdot \vec{v_1} \hat{n} \cdot \vec{v_2} \vec{v_1} \cdot \vec{v_1} - 6 \hat{n} \times \vec{S_1} \cdot \vec{a_1} \hat{n} \cdot \vec{v_2} \vec{v_1} \cdot \vec{v_1} - 16 \vec{S_1} \times \vec{v_1} \cdot \vec{v_2} \vec{v_1} \cdot \vec{v_2} - 16 \vec{S_1} \times \vec{a_1} \cdot \vec{v_2} \vec{v_1} \cdot \vec{v_2} + \\ & 6 \vec{S_1} \times \vec{v_1} \cdot \vec{a_1} \vec{v_1} \cdot \vec{v_2} + 16 \hat{n} \times \vec{S_1} \cdot \vec{v_1} \hat{n} \cdot \vec{v_2} \vec{v_1} \cdot \vec{v_2} + 16 \hat{n} \times \vec{S_1} \cdot \vec{a_1} \hat{n} \cdot \vec{v_2} \vec{v_1} \cdot \vec{v_2} - 2 \vec{S_1} \times \vec{v_1} \cdot \vec{v_2} \vec{v_2} \cdot \vec{a_2} + \\ & 3 \vec{S_1} \times \vec{v_1} \cdot \vec{v_2} \vec{v_2} \cdot \vec{v_2} + \vec{S_1} \times \vec{a_1} \cdot \vec{v_2} \vec{v_2} \cdot \vec{v_2} - \vec{S_1} \times \vec{v_1} \cdot \vec{a_2} \vec{v_2} \cdot \vec{v_2} - \hat{n} \times \vec{S_1} \cdot \vec{v_1} \hat{n} \cdot \vec{v_2} \vec{v_2} \cdot \vec{v_2} - 3 \hat{n} \times \vec{S_1} \cdot \vec{a_1} \hat{n} \cdot \vec{v_2} \vec{v_2} \cdot \vec{v_2} \Big) \\ & m_1 m_2 G^2 + \frac{1}{r^3} \Big( -12 \vec{S_1} \times \vec{v_1} \cdot \vec{v_2} (\hat{n} \cdot \vec{v_1})^3 - 12 \vec{S_1} \times \vec{v_1} \cdot \vec{v_2} \hat{n} \cdot \vec{v_2} (\hat{n} \cdot \vec{v_1})^2 - 12 \hat{n} \times \vec{S_1} \cdot \vec{v_2} \vec{v_1} \cdot \vec{v_1} (\hat{n} \cdot \vec{v_1})^2 - \\ & 52 \hat{n} \times \vec{S_1} \cdot \vec{v_1} \vec{v_1} \cdot \vec{v_2} (\hat{n} \cdot \vec{v_1})^2 - 12 \hat{n} \times \vec{S_1} \cdot \vec{v_2} \vec{v_2} \cdot \vec{v_2} (\hat{n} \cdot \vec{v_1})^2 - \vec{S_1} \times \vec{v_1} \cdot \vec{v_2} \vec{v_1} \cdot \vec{v_1} \hat{n} \cdot \vec{v_1} + \\ & 16 \hat{n} \times \vec{S_1} \cdot \vec{v_1} \hat{n} \cdot \vec{v_2} \vec{v_1} \cdot \vec{v_1} \hat{n} \cdot \vec{v_1} - 12 \hat{n} \times \vec{S_1} \cdot \vec{v_2} \hat{n} \cdot \vec{v_2} \vec{v_1} \cdot \vec{v_1} \hat{n} \cdot \vec{v_1} + 19 \vec{S_1} \times \vec{v_1} \cdot \vec{v_2} \vec{v_1} \cdot \vec{v_2} \hat{n} \cdot \vec{v_1} - \\ & 52 \hat{n} \times \vec{S_1} \cdot \vec{v_1} \hat{n} \cdot \vec{v_2} \vec{v_1} \cdot \vec{v_2} \hat{n} \cdot \vec{v_1} - 6 \vec{S_1} \times \vec{v_1} \cdot \vec{v_2} \vec{v_2} \cdot \vec{v_2} \hat{n} \cdot \vec{v_1} + 4 \hat{n} \times \vec{S_1} \cdot \vec{v_1} \hat{n} \cdot \vec{v_2} \vec{v_2} \cdot \vec{v_2} \hat{n} \cdot \vec{v_1} - \\ & 12 \hat{n} \times \vec{S_1} \cdot \vec{v_2} \hat{n} \cdot \vec{v_2} \vec{v_2} \cdot \vec{v_2} \hat{n} \cdot \vec{v_1} + 3 \hat{n} \times \vec{S_1} \cdot \vec{v_2} (\vec{v_1} \cdot \vec{v_1})^2 + 13 \hat{n} \times \vec{S_1} \cdot \vec{v_1} (\vec{v_1} \cdot \vec{v_2})^2 + \\ & 5 \hat{n} \times \vec{S_1} \cdot \vec{v_1} \vec{v_1} \cdot \vec{v_1} \vec{v_1} \cdot \vec{v_2} + 3 \hat{n} \times \vec{S_1} \cdot \vec{v_2} \vec{v_1} \cdot \vec{v_1} \vec{v_1} \cdot \vec{v_2} - 2 \vec{S_1} \times \vec{v_1} \cdot \vec{v_2} \hat{n} \cdot \vec{v_2} \vec{v_2} \cdot \vec{v_2} + \\ & 3 \hat{n} \times \vec{S_1} \cdot \vec{v_2} \vec{v_1} \cdot \vec{v_1} \vec{v_2} \cdot \vec{v_2} - 3 \hat{n} \times \vec{S_1} \cdot \vec{v_1} \vec{v_1} \cdot \vec{v_2} \vec{v_2} \cdot \vec{v_2} + 3 \hat{n} \times \vec{S_1} \cdot \vec{v_2} \vec{v_1} \cdot \vec{v_2} \vec{v_2} \cdot \vec{v_2} \Big) m_1 m_2 G^2 \Big\} \end{aligned}$$

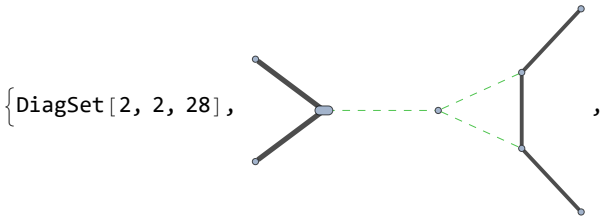

$$\begin{aligned} & \frac{1}{r} G^2 \left( 8 \vec{a}_1 \times \vec{S}_1 \cdot \vec{v}_2 \hat{n} \cdot \vec{v}_2 - 8 \vec{S}_1 \times \vec{v}_1 \cdot \vec{v}_2 \hat{n} \cdot \vec{v}_2 + 16 \vec{a}_1 \times \vec{S}_1 \cdot \vec{v}_2 \hat{n} \cdot \vec{v}_2 + \right. \\ & \quad \left. 16 \vec{a}_1 \times \vec{a}_2 \cdot \vec{S}_1 \hat{n} \cdot \vec{v}_2 + 16 \vec{a}_2 \times \vec{S}_1 \cdot \vec{v}_1 \hat{n} \cdot \vec{v}_2 - 8 \hat{n} \times \vec{S}_1 \cdot \vec{v}_1 \vec{a}_2 \cdot \vec{v}_2 + 8 \hat{n} \times \vec{a}_1 \cdot \vec{S}_1 \vec{a}_2 \cdot \vec{v}_2 \right) m_2^2 + \frac{1}{r^2} \\ & G^2 \left( 16 \vec{S}_1 \times \vec{v}_1 \cdot \vec{v}_2 (\hat{n} \cdot \vec{v}_2)^2 - 16 \vec{a}_1 \times \vec{S}_1 \cdot \vec{v}_2 (\hat{n} \cdot \vec{v}_2)^2 + 4 \vec{S}_1 \times \vec{v}_1 \cdot \vec{v}_2 \hat{n} \cdot \vec{a}_1 \hat{n} \cdot \vec{v}_2 + 20 \vec{S}_1 \times \vec{v}_1 \cdot \vec{v}_2 \hat{n} \cdot \vec{v}_1 \hat{n} \cdot \vec{v}_2 - \right. \\ & \quad 20 \vec{a}_1 \times \vec{S}_1 \cdot \vec{v}_2 \hat{n} \cdot \vec{v}_1 \hat{n} \cdot \vec{v}_2 - 8 \vec{a}_2 \times \vec{S}_1 \cdot \vec{v}_1 \hat{n} \cdot \vec{v}_1 \hat{n} \cdot \vec{v}_2 + 12 \hat{n} \times \vec{S}_1 \cdot \vec{v}_1 \vec{a}_1 \cdot \vec{v}_2 \hat{n} \cdot \vec{v}_2 - 24 \hat{n} \times \vec{S}_1 \cdot \vec{v}_1 \vec{a}_2 \cdot \vec{v}_1 \hat{n} \cdot \vec{v}_2 - \\ & \quad 16 \hat{n} \times \vec{S}_1 \cdot \vec{v}_2 \vec{a}_2 \cdot \vec{v}_2 \hat{n} \cdot \vec{v}_2 + 12 \hat{n} \times \vec{S}_1 \cdot \vec{v}_1 \vec{v}_1 \cdot \vec{v}_2 \hat{n} \cdot \vec{v}_2 - 12 \hat{n} \times \vec{a}_1 \cdot \vec{S}_1 \vec{v}_1 \cdot \vec{v}_2 \hat{n} \cdot \vec{v}_2 - 4 \hat{n} \times \vec{S}_1 \cdot \vec{v}_1 \vec{v}_2 \cdot \vec{v}_2 \hat{n} \cdot \vec{v}_2 + \\ & \quad 8 \hat{n} \times \vec{S}_1 \cdot \vec{v}_2 \vec{v}_2 \cdot \vec{v}_2 \hat{n} \cdot \vec{v}_2 + 4 \hat{n} \times \vec{a}_1 \cdot \vec{S}_1 \vec{v}_2 \cdot \vec{v}_2 \hat{n} \cdot \vec{v}_2 + 16 \hat{n} \times \vec{a}_2 \cdot \vec{S}_1 \vec{v}_2 \cdot \vec{v}_2 \hat{n} \cdot \vec{v}_2 - 8 \vec{S}_1 \times \vec{v}_1 \cdot \vec{v}_2 \vec{a}_1 \cdot \vec{v}_2 + \\ & \quad 12 \vec{S}_1 \times \vec{v}_1 \cdot \vec{v}_2 \vec{a}_2 \cdot \vec{v}_1 + 16 \hat{n} \times \vec{S}_1 \cdot \vec{v}_1 \hat{n} \cdot \vec{v}_1 \vec{a}_2 \cdot \vec{v}_2 - 16 \vec{S}_1 \times \vec{v}_1 \cdot \vec{v}_2 \vec{v}_1 \cdot \vec{v}_2 + 16 \vec{a}_1 \times \vec{S}_1 \cdot \vec{v}_2 \vec{v}_1 \cdot \vec{v}_2 + \\ & \quad \left. 4 \vec{a}_2 \times \vec{S}_1 \cdot \vec{v}_1 \vec{v}_1 \cdot \vec{v}_2 - 4 \vec{S}_1 \times \vec{v}_1 \cdot \vec{v}_2 \vec{v}_2 \cdot \vec{v}_2 + 4 \vec{a}_1 \times \vec{S}_1 \cdot \vec{v}_2 \vec{v}_2 \cdot \vec{v}_2 - 8 \vec{a}_2 \times \vec{S}_1 \cdot \vec{v}_2 \vec{v}_2 \cdot \vec{v}_2 \right) m_2^2 + \\ & \frac{1}{r^3} G^2 \left( -16 \vec{S}_1 \times \vec{v}_1 \cdot \vec{v}_2 \hat{n} \cdot \vec{v}_2 (\hat{n} \cdot \vec{v}_1)^2 - 16 \vec{S}_1 \times \vec{v}_1 \cdot \vec{v}_2 (\hat{n} \cdot \vec{v}_2)^2 \hat{n} \cdot \vec{v}_1 + 20 \vec{S}_1 \times \vec{v}_1 \cdot \vec{v}_2 \vec{v}_1 \cdot \vec{v}_2 \hat{n} \cdot \vec{v}_1 - \right. \\ & \quad 48 \hat{n} \times \vec{S}_1 \cdot \vec{v}_1 \hat{n} \cdot \vec{v}_2 \vec{v}_1 \cdot \vec{v}_2 \hat{n} \cdot \vec{v}_1 - \vec{S}_1 \times \vec{v}_1 \cdot \vec{v}_2 \vec{v}_2 \cdot \vec{v}_2 \hat{n} \cdot \vec{v}_1 + 16 \hat{n} \times \vec{S}_1 \cdot \vec{v}_1 \hat{n} \cdot \vec{v}_2 \vec{v}_2 \cdot \vec{v}_2 \hat{n} \cdot \vec{v}_1 - \\ & \quad 32 \hat{n} \times \vec{S}_1 \cdot \vec{v}_2 \hat{n} \cdot \vec{v}_2 \vec{v}_2 \cdot \vec{v}_2 \hat{n} \cdot \vec{v}_1 + 12 \hat{n} \times \vec{S}_1 \cdot \vec{v}_1 (\vec{v}_1 \cdot \vec{v}_2)^2 + 6 \hat{n} \times \vec{S}_1 \cdot \vec{v}_2 (\vec{v}_2 \cdot \vec{v}_2)^2 + 4 \vec{S}_1 \times \vec{v}_1 \cdot \vec{v}_2 \hat{n} \cdot \vec{v}_2 \vec{v}_1 \cdot \vec{v}_1 - \\ & \quad 48 \hat{n} \times \vec{S}_1 \cdot \vec{v}_1 (\hat{n} \cdot \vec{v}_2)^2 \vec{v}_1 \cdot \vec{v}_2 + 32 \vec{S}_1 \times \vec{v}_1 \cdot \vec{v}_2 \hat{n} \cdot \vec{v}_2 \vec{v}_1 \cdot \vec{v}_2 - 32 \hat{n} \times \vec{S}_1 \cdot \vec{v}_2 (\hat{n} \cdot \vec{v}_2)^2 \vec{v}_2 \cdot \vec{v}_2 - \\ & \quad \left. 8 \vec{S}_1 \times \vec{v}_1 \cdot \vec{v}_2 \hat{n} \cdot \vec{v}_2 \vec{v}_2 \cdot \vec{v}_2 + 5 \hat{n} \times \vec{S}_1 \cdot \vec{v}_1 \vec{v}_1 \cdot \vec{v}_2 \vec{v}_2 \cdot \vec{v}_2 + 8 \hat{n} \times \vec{S}_1 \cdot \vec{v}_2 \vec{v}_1 \cdot \vec{v}_2 \vec{v}_2 \cdot \vec{v}_2 \right) m_2^2 \} \end{aligned}$$

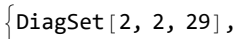

$$\left(\frac{8}{3} \hat{n} \times \vec{S_1} \cdot \vec{v_2} \left(\hat{n} \cdot \vec{v_1}\right)^3 + \frac{10}{3} \hat{n} \times \vec{S_1} \cdot \vec{a_2} \left(\hat{n} \cdot \vec{v_1}\right)^3 + 8 \vec{S_1} \times \vec{v_1} \cdot \vec{v_2} \left(\hat{n} \cdot \vec{v_1}\right)^2 + \frac{16}{3} \vec{S_1} \times \vec{a_1} \cdot \vec{v_2} \left(\hat{n} \cdot \vec{v_1}\right)^2 + \right.$$



$$\begin{aligned}
& \frac{4}{3} \hat{n} \times \vec{S}_1 \cdot \vec{v}_2 \vec{v}_2 \cdot \vec{v}_2 \hat{n} \cdot \vec{v}_1 - \hat{n} \times \vec{S}_1 \cdot \vec{a}_1 \vec{v}_2 \cdot \vec{v}_2 \hat{n} \cdot \vec{v}_1 - \frac{16}{3} \vec{S}_1 \times \vec{v}_1 \cdot \vec{v}_2 (\hat{n} \cdot \vec{v}_2)^2 - \frac{4}{3} \vec{S}_1 \times \vec{v}_1 \cdot \vec{a}_1 (\hat{n} \cdot \vec{v}_2)^2 + \\
& \frac{4}{3} \hat{n} \times \vec{S}_1 \cdot \vec{v}_1 \hat{n} \cdot \vec{a}_1 (\hat{n} \cdot \vec{v}_2)^2 + \vec{S}_1 \times \vec{v}_1 \cdot \vec{v}_2 \hat{n} \cdot \vec{a}_1 \hat{n} \cdot \vec{v}_2 - \vec{S}_1 \times \vec{v}_1 \cdot \vec{v}_2 \vec{a}_1 \cdot \vec{v}_2 + \frac{1}{3} \hat{n} \times \vec{S}_1 \cdot \vec{v}_1 \hat{n} \cdot \vec{v}_2 \vec{a}_1 \cdot \vec{v}_2 - \\
& \vec{S}_1 \times \vec{v}_1 \cdot \vec{v}_2 \vec{v}_1 \cdot \vec{a}_1 - \frac{2}{3} \hat{n} \times \vec{S}_1 \cdot \vec{v}_1 \hat{n} \cdot \vec{v}_2 \vec{v}_1 \cdot \vec{a}_1 - \frac{2}{3} \hat{n} \times \vec{S}_1 \cdot \vec{v}_2 \hat{n} \cdot \vec{v}_2 \vec{v}_1 \cdot \vec{a}_1 - 6 \vec{S}_1 \times \vec{v}_1 \cdot \vec{v}_2 \vec{v}_1 \cdot \vec{a}_2 + \\
& 8 \hat{n} \times \vec{S}_1 \cdot \vec{v}_1 \hat{n} \cdot \vec{v}_2 \vec{v}_1 \cdot \vec{a}_2 - 2 \vec{S}_1 \times \vec{v}_1 \cdot \vec{v}_2 \vec{v}_1 \cdot \vec{v}_1 - \frac{11}{3} \vec{S}_1 \times \vec{a}_1 \cdot \vec{v}_2 \vec{v}_1 \cdot \vec{v}_1 - \frac{8}{3} \vec{S}_1 \times \vec{v}_1 \cdot \vec{a}_2 \vec{v}_1 \cdot \vec{v}_1 - \\
& \vec{S}_1 \times \vec{v}_2 \cdot \vec{a}_2 \vec{v}_1 \cdot \vec{v}_1 - \frac{7}{3} \hat{n} \times \vec{S}_1 \cdot \vec{v}_2 \hat{n} \cdot \vec{a}_1 \vec{v}_1 \cdot \vec{v}_1 + \frac{1}{3} \hat{n} \times \vec{S}_1 \cdot \vec{v}_1 \hat{n} \cdot \vec{a}_2 \vec{v}_1 \cdot \vec{v}_1 - 2 \hat{n} \times \vec{S}_1 \cdot \vec{v}_2 \hat{n} \cdot \vec{a}_2 \vec{v}_1 \cdot \vec{v}_1 + \\
& \frac{10}{3} \hat{n} \times \vec{S}_1 \cdot \vec{v}_2 \hat{n} \cdot \vec{v}_2 \vec{v}_1 \cdot \vec{v}_1 - 4 \hat{n} \times \vec{S}_1 \cdot \vec{a}_2 \hat{n} \cdot \vec{v}_2 \vec{v}_1 \cdot \vec{v}_1 + \frac{16}{3} \vec{S}_1 \times \vec{v}_1 \cdot \vec{v}_2 \vec{v}_1 \cdot \vec{v}_2 + \frac{11}{3} \vec{S}_1 \times \vec{a}_1 \cdot \vec{v}_2 \vec{v}_1 \cdot \vec{v}_2 - \\
& \frac{5}{3} \vec{S}_1 \times \vec{v}_1 \cdot \vec{a}_1 \vec{v}_1 \cdot \vec{v}_2 - 6 \vec{S}_1 \times \vec{v}_1 \cdot \vec{a}_2 \vec{v}_1 \cdot \vec{v}_2 + \frac{13}{3} \hat{n} \times \vec{S}_1 \cdot \vec{v}_1 \hat{n} \cdot \vec{a}_1 \vec{v}_1 \cdot \vec{v}_2 + \frac{1}{3} \hat{n} \times \vec{S}_1 \cdot \vec{v}_2 \hat{n} \cdot \vec{a}_1 \vec{v}_1 \cdot \vec{v}_2 + \\
& 4 \hat{n} \times \vec{S}_1 \cdot \vec{v}_1 \hat{n} \cdot \vec{a}_2 \vec{v}_1 \cdot \vec{v}_2 + \hat{n} \times \vec{S}_1 \cdot \vec{v}_1 \hat{n} \cdot \vec{v}_2 \vec{v}_1 \cdot \vec{v}_2 + \frac{8}{3} \hat{n} \times \vec{S}_1 \cdot \vec{v}_2 \hat{n} \cdot \vec{v}_2 \vec{v}_1 \cdot \vec{v}_2 - 3 \hat{n} \times \vec{S}_1 \cdot \vec{a}_1 \hat{n} \cdot \vec{v}_2 \vec{v}_1 \cdot \vec{v}_2 + \\
& \frac{8}{3} \vec{S}_1 \times \vec{v}_1 \cdot \vec{v}_2 \vec{v}_2 \cdot \vec{v}_2 + \frac{2}{3} \vec{S}_1 \times \vec{v}_1 \cdot \vec{a}_1 \vec{v}_2 \cdot \vec{v}_2 - \frac{1}{3} \hat{n} \times \vec{S}_1 \cdot \vec{v}_1 \hat{n} \cdot \vec{a}_1 \vec{v}_2 \cdot \vec{v}_2 \Big) m_1 m_2 G^2 + \frac{1}{r^3} \\
& \left( -4 \hat{n} \times \vec{S}_1 \cdot \vec{v}_2 (\hat{n} \cdot \vec{v}_1)^4 - \frac{17}{3} \vec{S}_1 \times \vec{v}_1 \cdot \vec{v}_2 (\hat{n} \cdot \vec{v}_1)^3 + 3 \hat{n} \times \vec{S}_1 \cdot \vec{v}_1 \hat{n} \cdot \vec{v}_2 (\hat{n} \cdot \vec{v}_1)^3 + 20 \hat{n} \times \vec{S}_1 \cdot \vec{v}_2 \hat{n} \cdot \vec{v}_2 (\hat{n} \cdot \vec{v}_1)^3 - \right. \\
& 8 \hat{n} \times \vec{S}_1 \cdot \vec{v}_1 (\hat{n} \cdot \vec{v}_2)^2 (\hat{n} \cdot \vec{v}_1)^2 + 24 \hat{n} \times \vec{S}_1 \cdot \vec{v}_2 (\hat{n} \cdot \vec{v}_2)^2 (\hat{n} \cdot \vec{v}_1)^2 + \frac{56}{3} \vec{S}_1 \times \vec{v}_1 \cdot \vec{v}_2 \hat{n} \cdot \vec{v}_2 (\hat{n} \cdot \vec{v}_1)^2 + \\
& 2 \hat{n} \times \vec{S}_1 \cdot \vec{v}_2 \vec{v}_1 \cdot \vec{v}_1 (\hat{n} \cdot \vec{v}_1)^2 - 7 \hat{n} \times \vec{S}_1 \cdot \vec{v}_1 \vec{v}_1 \cdot \vec{v}_2 (\hat{n} \cdot \vec{v}_1)^2 - 10 \hat{n} \times \vec{S}_1 \cdot \vec{v}_2 \vec{v}_1 \cdot \vec{v}_2 (\hat{n} \cdot \vec{v}_1)^2 + \\
& \frac{4}{3} \hat{n} \times \vec{S}_1 \cdot \vec{v}_1 \vec{v}_2 \cdot \vec{v}_2 (\hat{n} \cdot \vec{v}_1)^2 - 4 \hat{n} \times \vec{S}_1 \cdot \vec{v}_2 \vec{v}_2 \cdot \vec{v}_2 (\hat{n} \cdot \vec{v}_1)^2 + 16 \vec{S}_1 \times \vec{v}_1 \cdot \vec{v}_2 (\hat{n} \cdot \vec{v}_2)^2 \hat{n} \cdot \vec{v}_1 + \\
& 5 \vec{S}_1 \times \vec{v}_1 \cdot \vec{v}_2 \vec{v}_1 \cdot \vec{v}_1 \hat{n} \cdot \vec{v}_1 - \hat{n} \times \vec{S}_1 \cdot \vec{v}_1 \hat{n} \cdot \vec{v}_2 \vec{v}_1 \cdot \vec{v}_1 \hat{n} \cdot \vec{v}_1 - 16 \hat{n} \times \vec{S}_1 \cdot \vec{v}_2 \hat{n} \cdot \vec{v}_2 \vec{v}_1 \cdot \vec{v}_1 \hat{n} \cdot \vec{v}_1 - \\
& \frac{25}{3} \vec{S}_1 \times \vec{v}_1 \cdot \vec{v}_2 \vec{v}_1 \cdot \vec{v}_2 \hat{n} \cdot \vec{v}_1 + \frac{4}{3} \hat{n} \times \vec{S}_1 \cdot \vec{v}_1 \hat{n} \cdot \vec{v}_2 \vec{v}_1 \cdot \vec{v}_2 \hat{n} \cdot \vec{v}_1 - 16 \hat{n} \times \vec{S}_1 \cdot \vec{v}_2 \hat{n} \cdot \vec{v}_2 \vec{v}_1 \cdot \vec{v}_2 \hat{n} \cdot \vec{v}_1 - \\
& 4 \vec{S}_1 \times \vec{v}_1 \cdot \vec{v}_2 \vec{v}_2 \cdot \vec{v}_2 \hat{n} \cdot \vec{v}_1 + \frac{1}{3} \hat{n} \times \vec{S}_1 \cdot \vec{v}_1 (\vec{v}_1 \cdot \vec{v}_2)^2 + 2 \hat{n} \times \vec{S}_1 \cdot \vec{v}_2 (\vec{v}_1 \cdot \vec{v}_2)^2 + \frac{4}{3} \hat{n} \times \vec{S}_1 \cdot \vec{v}_1 (\hat{n} \cdot \vec{v}_2)^2 \vec{v}_1 \cdot \vec{v}_1 - \\
& 8 \hat{n} \times \vec{S}_1 \cdot \vec{v}_2 (\hat{n} \cdot \vec{v}_2)^2 \vec{v}_1 \cdot \vec{v}_1 - \frac{17}{3} \vec{S}_1 \times \vec{v}_1 \cdot \vec{v}_2 \hat{n} \cdot \vec{v}_2 \vec{v}_1 \cdot \vec{v}_1 + 16 \hat{n} \times \vec{S}_1 \cdot \vec{v}_1 (\hat{n} \cdot \vec{v}_2)^2 \vec{v}_1 \cdot \vec{v}_2 - \\
& 16 \vec{S}_1 \times \vec{v}_1 \cdot \vec{v}_2 \hat{n} \cdot \vec{v}_2 \vec{v}_1 \cdot \vec{v}_2 - \hat{n} \times \vec{S}_1 \cdot \vec{v}_1 \vec{v}_1 \cdot \vec{v}_1 \vec{v}_1 \cdot \vec{v}_2 + 4 \hat{n} \times \vec{S}_1 \cdot \vec{v}_2 \vec{v}_1 \cdot \vec{v}_1 \vec{v}_1 \cdot \vec{v}_2 - \\
& \frac{1}{3} \hat{n} \times \vec{S}_1 \cdot \vec{v}_1 \vec{v}_1 \cdot \vec{v}_1 \vec{v}_2 \cdot \vec{v}_2 + 2 \hat{n} \times \vec{S}_1 \cdot \vec{v}_2 \vec{v}_1 \cdot \vec{v}_1 \vec{v}_2 \cdot \vec{v}_2 - 4 \hat{n} \times \vec{S}_1 \cdot \vec{v}_1 \vec{v}_1 \cdot \vec{v}_2 \vec{v}_2 \cdot \vec{v}_2 \Big) m_1 m_2 G^2 + \\
& m_1 m_2 \left( -\frac{8}{3} \log\left(\frac{r}{R_\theta}\right) \vec{S}_1 \times \vec{a}_1 \cdot \vec{v}_2 + \frac{10}{9} \vec{S}_1 \times \vec{a}_1 \cdot \vec{v}_2 - \frac{10}{9} \vec{S}_1 \times \vec{v}_1 \cdot \vec{a}_2 - \frac{2}{3} \vec{S}_1 \times \vec{a}_1 \cdot \vec{v}_2 - \frac{2}{3} \vec{S}_1 \times \vec{v}_1 \cdot \vec{a}_2 - \frac{2}{3} \hat{n} \times \vec{S}_1 \cdot \vec{a}_2 \hat{n} \cdot \vec{a}_1 + \right. \\
& \frac{4}{3} \hat{n} \times \vec{S}_1 \cdot \vec{v}_2 \hat{n} \cdot \vec{a}_1 - \frac{2}{3} \hat{n} \times \vec{S}_1 \cdot \vec{a}_1 \hat{n} \cdot \vec{a}_2 - \frac{2}{3} \hat{n} \times \vec{S}_1 \cdot \vec{v}_1 \hat{n} \cdot \vec{a}_2 - \frac{2}{3} \hat{n} \times \vec{S}_1 \cdot \vec{a}_2 \hat{n} \cdot \vec{v}_1 + \frac{4}{3} \hat{n} \times \vec{S}_1 \cdot \vec{a}_2 \hat{n} \cdot \vec{v}_1 - \\
& \left. \frac{2}{3} \hat{n} \times \vec{S}_1 \cdot \vec{a}_1 \hat{n} \cdot \vec{v}_2 - \frac{2}{3} \hat{n} \times \vec{S}_1 \cdot \vec{a}_1 \hat{n} \cdot \vec{v}_2 + \frac{8}{3} \vec{S}_1 \times \vec{v}_1 \cdot \vec{a}_2 \log\left(\frac{r}{R_\theta}\right) + \frac{\frac{4}{3} \vec{S}_1 \times \vec{a}_1 \cdot \vec{v}_2 - \frac{4}{3} \vec{S}_1 \times \vec{v}_1 \cdot \vec{a}_2}{\epsilon_d} \right) G^2 \Big\}
\end{aligned}$$

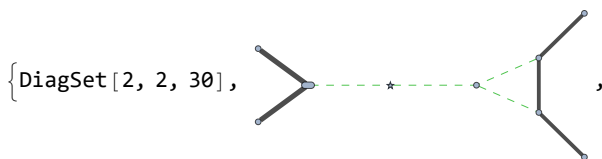

$$\frac{1}{r} G^2 \left( \frac{8}{3} \hat{n} \times \vec{S}_1 \cdot \vec{v}_2 (\hat{n} \cdot \vec{v}_2)^2 + 8 \hat{n} \times \vec{a}_2 \cdot \vec{S}_1 (\hat{n} \cdot \vec{v}_2)^2 + \frac{8}{3} \vec{a}_2 \times \vec{S}_1 \cdot \vec{v}_1 \hat{n} \cdot \vec{v}_2 - \frac{4}{3} \vec{a}_1 \times \vec{a}_2 \cdot \vec{S}_1 \hat{n} \cdot \vec{v}_2 - \frac{8}{3} \vec{a}_2 \times \vec{S}_1 \cdot \vec{v}_1 \hat{n} \cdot \vec{v}_2 - \right.$$

$$\begin{aligned}
& \frac{16}{3} \vec{a}_2 \times \vec{S}_1 \cdot \vec{v}_2 \hat{n} \cdot \vec{v}_2 + \frac{8}{3} \hat{n} \times \vec{a}_2 \cdot \vec{S}_1 \hat{n} \cdot \vec{a}_1 \hat{n} \cdot \vec{v}_2 - \frac{16}{3} \hat{n} \times \vec{S}_1 \cdot \vec{v}_2 \hat{n} \cdot \vec{a}_2 \hat{n} \cdot \vec{v}_2 - \frac{16}{3} \hat{n} \times \vec{a}_2 \cdot \vec{S}_1 \hat{n} \cdot \vec{v}_1 \hat{n} \cdot \vec{v}_2 + \\
& \frac{16}{3} \hat{n} \times \vec{a}_2 \cdot \vec{S}_1 \hat{n} \cdot \vec{v}_1 \hat{n} \cdot \vec{v}_2 - \frac{8}{3} \vec{S}_1 \times \vec{v}_1 \cdot \vec{v}_2 \hat{n} \cdot \vec{a}_2 + \frac{4}{3} \vec{a}_1 \times \vec{S}_1 \cdot \vec{v}_2 \hat{n} \cdot \vec{a}_2 + \frac{8}{3} \vec{a}_2 \times \vec{S}_1 \cdot \vec{v}_1 \hat{n} \cdot \vec{a}_2 - \\
& \frac{8}{3} \hat{n} \times \vec{S}_1 \cdot \vec{v}_2 \hat{n} \cdot \vec{a}_1 \hat{n} \cdot \vec{a}_2 + \frac{8}{3} \vec{a}_2 \times \vec{S}_1 \cdot \vec{v}_2 \hat{n} \cdot \vec{v}_1 - \frac{16}{3} \hat{n} \times \vec{S}_1 \cdot \vec{v}_2 \hat{n} \cdot \vec{a}_2 \hat{n} \cdot \vec{v}_1 - \frac{16}{3} \hat{n} \times \vec{a}_2 \cdot \vec{S}_1 \hat{n} \cdot \vec{a}_2 \hat{n} \cdot \vec{v}_1 + \\
& \frac{4}{3} \hat{n} \times \vec{S}_1 \cdot \vec{v}_2 \vec{a}_1 \cdot \vec{a}_2 - \frac{4}{3} \hat{n} \times \vec{a}_2 \cdot \vec{S}_1 \vec{a}_1 \cdot \vec{v}_2 + \frac{8}{3} \hat{n} \times \vec{S}_1 \cdot \vec{v}_2 \vec{a}_2 \cdot \vec{v}_1 + \frac{8}{3} \hat{n} \times \vec{a}_2 \cdot \vec{S}_1 \vec{a}_2 \cdot \vec{v}_1 + \frac{2}{3} \hat{n} \times \vec{S}_1 \cdot \vec{v}_2 \vec{a}_2 \cdot \vec{v}_2 + \\
& \frac{8}{3} \hat{n} \times \vec{a}_2 \cdot \vec{S}_1 \vec{v}_1 \cdot \vec{v}_2 - \frac{8}{3} \hat{n} \times \vec{a}_2 \cdot \vec{S}_1 \vec{v}_1 \cdot \vec{v}_2 - \frac{4}{3} \hat{n} \times \vec{S}_1 \cdot \vec{v}_2 \vec{v}_2 \cdot \vec{v}_2 - 3 \hat{n} \times \vec{a}_2 \cdot \vec{S}_1 \vec{v}_2 \cdot \vec{v}_2 \Big) m_2^2 + \frac{1}{r^2} \\
& G^2 \left( -\frac{32}{3} \hat{n} \times \vec{S}_1 \cdot \vec{v}_2 (\hat{n} \cdot \vec{v}_2)^3 - \frac{16}{3} \vec{S}_1 \times \vec{v}_1 \cdot \vec{v}_2 (\hat{n} \cdot \vec{v}_2)^2 + \frac{8}{3} \vec{a}_1 \times \vec{S}_1 \cdot \vec{v}_2 (\hat{n} \cdot \vec{v}_2)^2 + 8 \vec{a}_2 \times \vec{S}_1 \cdot \vec{v}_1 (\hat{n} \cdot \vec{v}_2)^2 - \right. \\
& \frac{32}{3} \hat{n} \times \vec{S}_1 \cdot \vec{v}_2 \hat{n} \cdot \vec{a}_1 (\hat{n} \cdot \vec{v}_2)^2 - \frac{64}{3} \hat{n} \times \vec{S}_1 \cdot \vec{v}_2 \hat{n} \cdot \vec{v}_1 (\hat{n} \cdot \vec{v}_2)^2 - 32 \hat{n} \times \vec{a}_2 \cdot \vec{S}_1 \hat{n} \cdot \vec{v}_1 (\hat{n} \cdot \vec{v}_2)^2 - \\
& \frac{32}{3} \hat{n} \times \vec{a}_2 \cdot \vec{S}_1 (\hat{n} \cdot \vec{v}_1)^2 \hat{n} \cdot \vec{v}_2 + \frac{16}{3} \vec{S}_1 \times \vec{v}_1 \cdot \vec{v}_2 \hat{n} \cdot \vec{a}_2 \hat{n} \cdot \vec{v}_2 + \frac{16}{3} \vec{a}_2 \times \vec{S}_1 \cdot \vec{v}_1 \hat{n} \cdot \vec{v}_1 \hat{n} \cdot \vec{v}_2 + \\
& \frac{32}{3} \vec{a}_2 \times \vec{S}_1 \cdot \vec{v}_2 \hat{n} \cdot \vec{v}_1 \hat{n} \cdot \vec{v}_2 + \frac{64}{3} \hat{n} \times \vec{S}_1 \cdot \vec{v}_2 \hat{n} \cdot \vec{a}_2 \hat{n} \cdot \vec{v}_1 \hat{n} \cdot \vec{v}_2 + \frac{16}{3} \hat{n} \times \vec{S}_1 \cdot \vec{v}_2 \vec{a}_1 \cdot \vec{v}_2 \hat{n} \cdot \vec{v}_2 - \\
& \frac{16}{3} \hat{n} \times \vec{S}_1 \cdot \vec{v}_2 \vec{a}_2 \cdot \vec{v}_1 \hat{n} \cdot \vec{v}_2 + \frac{8}{3} \hat{n} \times \vec{a}_2 \cdot \vec{S}_1 \vec{v}_1 \cdot \vec{v}_1 \hat{n} \cdot \vec{v}_2 + \frac{32}{3} \hat{n} \times \vec{S}_1 \cdot \vec{v}_2 \vec{v}_1 \cdot \vec{v}_2 \hat{n} \cdot \vec{v}_2 + \\
& 16 \hat{n} \times \vec{a}_2 \cdot \vec{S}_1 \vec{v}_1 \cdot \vec{v}_2 \hat{n} \cdot \vec{v}_2 + 6 \hat{n} \times \vec{S}_1 \cdot \vec{v}_2 \vec{v}_2 \cdot \vec{v}_2 \hat{n} \cdot \vec{v}_2 + \frac{32}{3} \hat{n} \times \vec{S}_1 \cdot \vec{v}_2 \hat{n} \cdot \vec{a}_2 (\hat{n} \cdot \vec{v}_1)^2 + \\
& \frac{16}{3} \vec{S}_1 \times \vec{v}_1 \cdot \vec{v}_2 \hat{n} \cdot \vec{a}_2 \hat{n} \cdot \vec{v}_1 - \frac{8}{3} \vec{S}_1 \times \vec{v}_1 \cdot \vec{v}_2 \vec{a}_2 \cdot \vec{v}_1 - \frac{16}{3} \hat{n} \times \vec{S}_1 \cdot \vec{v}_2 \hat{n} \cdot \vec{v}_1 \vec{a}_2 \cdot \vec{v}_1 - \frac{2}{3} \vec{S}_1 \times \vec{v}_1 \cdot \vec{v}_2 \vec{a}_2 \cdot \vec{v}_2 - \\
& \frac{4}{3} \hat{n} \times \vec{S}_1 \cdot \vec{v}_2 \hat{n} \cdot \vec{v}_1 \vec{a}_2 \cdot \vec{v}_2 - \frac{8}{3} \hat{n} \times \vec{S}_1 \cdot \vec{v}_2 \hat{n} \cdot \vec{a}_2 \vec{v}_1 \cdot \vec{v}_1 - \frac{8}{3} \vec{a}_2 \times \vec{S}_1 \cdot \vec{v}_1 \vec{v}_1 \cdot \vec{v}_2 - \frac{16}{3} \vec{a}_2 \times \vec{S}_1 \cdot \vec{v}_2 \vec{v}_1 \cdot \vec{v}_2 - \\
& \frac{16}{3} \hat{n} \times \vec{S}_1 \cdot \vec{v}_2 \hat{n} \cdot \vec{a}_2 \vec{v}_1 \cdot \vec{v}_2 + \frac{16}{3} \hat{n} \times \vec{a}_2 \cdot \vec{S}_1 \hat{n} \cdot \vec{v}_1 \vec{v}_1 \cdot \vec{v}_2 + \frac{8}{3} \vec{S}_1 \times \vec{v}_1 \cdot \vec{v}_2 \vec{v}_2 \cdot \vec{v}_2 - \frac{4}{3} \vec{a}_1 \times \vec{S}_1 \cdot \vec{v}_2 \vec{v}_2 \cdot \vec{v}_2 - \\
& 3 \vec{a}_2 \times \vec{S}_1 \cdot \vec{v}_1 \vec{v}_2 \cdot \vec{v}_2 + \frac{8}{3} \hat{n} \times \vec{S}_1 \cdot \vec{v}_2 \hat{n} \cdot \vec{a}_1 \vec{v}_2 \cdot \vec{v}_2 + \frac{16}{3} \hat{n} \times \vec{S}_1 \cdot \vec{v}_2 \hat{n} \cdot \vec{v}_1 \vec{v}_2 \cdot \vec{v}_2 + 6 \hat{n} \times \vec{a}_2 \cdot \vec{S}_1 \hat{n} \cdot \vec{v}_1 \vec{v}_2 \cdot \vec{v}_2 \Big) m_2^2 + \\
& \frac{1}{r^3} G^2 \left( \frac{32}{3} \vec{S}_1 \times \vec{v}_1 \cdot \vec{v}_2 (\hat{n} \cdot \vec{v}_2)^3 + 64 \hat{n} \times \vec{S}_1 \cdot \vec{v}_2 \hat{n} \cdot \vec{v}_1 (\hat{n} \cdot \vec{v}_2)^3 + 64 \hat{n} \times \vec{S}_1 \cdot \vec{v}_2 (\hat{n} \cdot \vec{v}_1)^2 (\hat{n} \cdot \vec{v}_2)^2 + \right. \\
& \frac{64}{3} \vec{S}_1 \times \vec{v}_1 \cdot \vec{v}_2 \hat{n} \cdot \vec{v}_1 (\hat{n} \cdot \vec{v}_2)^2 - \frac{32}{3} \hat{n} \times \vec{S}_1 \cdot \vec{v}_2 \vec{v}_1 \cdot \vec{v}_1 (\hat{n} \cdot \vec{v}_2)^2 - 32 \hat{n} \times \vec{S}_1 \cdot \vec{v}_2 \vec{v}_1 \cdot \vec{v}_2 (\hat{n} \cdot \vec{v}_2)^2 - \\
& \frac{32}{3} \vec{S}_1 \times \vec{v}_1 \cdot \vec{v}_2 \vec{v}_1 \cdot \vec{v}_2 \hat{n} \cdot \vec{v}_2 - \frac{128}{3} \hat{n} \times \vec{S}_1 \cdot \vec{v}_2 \hat{n} \cdot \vec{v}_1 \vec{v}_1 \cdot \vec{v}_2 \hat{n} \cdot \vec{v}_2 - 6 \vec{S}_1 \times \vec{v}_1 \cdot \vec{v}_2 \vec{v}_2 \cdot \vec{v}_2 \hat{n} \cdot \vec{v}_2 - \\
& 24 \hat{n} \times \vec{S}_1 \cdot \vec{v}_2 \hat{n} \cdot \vec{v}_1 \vec{v}_2 \cdot \vec{v}_2 \hat{n} \cdot \vec{v}_2 + \frac{16}{3} \hat{n} \times \vec{S}_1 \cdot \vec{v}_2 (\vec{v}_1 \cdot \vec{v}_2)^2 - \frac{32}{3} \hat{n} \times \vec{S}_1 \cdot \vec{v}_2 (\hat{n} \cdot \vec{v}_1)^2 \vec{v}_2 \cdot \vec{v}_2 - \\
& \frac{16}{3} \vec{S}_1 \times \vec{v}_1 \cdot \vec{v}_2 \hat{n} \cdot \vec{v}_1 \vec{v}_2 \cdot \vec{v}_2 + \frac{8}{3} \hat{n} \times \vec{S}_1 \cdot \vec{v}_2 \vec{v}_1 \cdot \vec{v}_1 \vec{v}_2 \cdot \vec{v}_2 + 6 \hat{n} \times \vec{S}_1 \cdot \vec{v}_2 \vec{v}_1 \cdot \vec{v}_2 \vec{v}_2 \cdot \vec{v}_2 \Big) m_2^2 + \\
& G^2 \left( \frac{8}{3} \log\left(\frac{r}{R_\theta}\right) \frac{1}{\vec{a}_2 \times \vec{S}_1 \cdot \vec{v}_2} - \frac{4 \frac{1}{\vec{a}_2} \times \frac{1}{\vec{S}_1} \cdot \vec{v}_2}{3 \in_d} - \frac{16}{9} \frac{1}{\vec{a}_2 \times \vec{S}_1 \cdot \vec{v}_2} + \frac{4}{3} \hat{n} \times \vec{S}_1 \cdot \vec{v}_2 \hat{n} \cdot \vec{a}_2 + \right. \\
& \left. \frac{8}{3} \hat{n} \times \vec{a}_2 \cdot \vec{S}_1 \hat{n} \cdot \vec{a}_2 + \frac{8}{3} \hat{n} \times \vec{a}_2 \cdot \vec{S}_1 \hat{n} \cdot \vec{v}_2 - \frac{4}{3} \hat{n} \times \vec{a}_2 \cdot \vec{S}_1 \hat{n} \cdot \vec{v}_2 \right) m_2^2 \Big\}
\end{aligned}$$

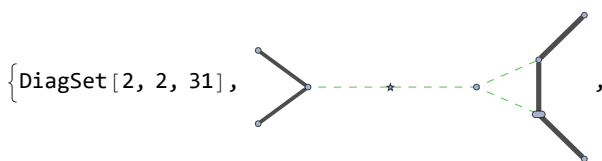

[illegible]

$$\begin{aligned}
& 2 \vec{S}_1 \times \vec{v}_1 \cdot \vec{v}_2 \vec{v}_2 \cdot \vec{v}_2 \hat{n} \cdot \vec{v}_1 - \frac{16}{3} \hat{n} \times \vec{S}_1 \cdot \vec{v}_1 (\vec{v}_1 \cdot \vec{v}_2)^2 + 4 \hat{n} \times \vec{S}_1 \cdot \vec{v}_2 (\vec{v}_1 \cdot \vec{v}_2)^2 + \frac{8}{3} \hat{n} \times \vec{S}_1 \cdot \vec{v}_1 (\hat{n} \cdot \vec{v}_2)^2 \vec{v}_1 \cdot \vec{v}_1 - \\
& 8 \hat{n} \times \vec{S}_1 \cdot \vec{v}_2 (\hat{n} \cdot \vec{v}_2)^2 \vec{v}_1 \cdot \vec{v}_1 - \frac{16}{3} \vec{S}_1 \times \vec{v}_1 \cdot \vec{v}_2 \hat{n} \cdot \vec{v}_2 \vec{v}_1 \cdot \vec{v}_1 - 4 \vec{S}_1 \times \vec{v}_1 \cdot \vec{v}_2 \hat{n} \cdot \vec{v}_2 \vec{v}_1 \cdot \vec{v}_2 + \\
& 6 \hat{n} \times \vec{S}_1 \cdot \vec{v}_2 \vec{v}_1 \cdot \vec{v}_1 \vec{v}_1 \cdot \vec{v}_2 - \frac{2}{3} \hat{n} \times \vec{S}_1 \cdot \vec{v}_1 \vec{v}_1 \cdot \vec{v}_1 \vec{v}_2 \cdot \vec{v}_2 + 2 \hat{n} \times \vec{S}_1 \cdot \vec{v}_2 \vec{v}_1 \cdot \vec{v}_1 \vec{v}_2 \cdot \vec{v}_2 \Big) m_1 m_2 G^2 + \\
& m_1 m_2 \left( -\frac{8}{3} \log\left(\frac{r}{R_\theta}\right) \frac{1}{\vec{S}_1 \times \vec{a}_1 \cdot \vec{a}_2} + \frac{16}{9} \frac{1}{\vec{S}_1 \times \vec{a}_1 \cdot \vec{a}_2} - \frac{1}{3} \frac{1}{\vec{S}_1 \times \vec{v}_1 \cdot \vec{a}_2} + \frac{13}{9} \frac{2}{\vec{S}_1 \times \vec{v}_1 \cdot \vec{a}_2} + \frac{1}{3} \frac{1}{\vec{S}_1 \times \vec{a}_1 \cdot \vec{a}_2} - \frac{1}{3} \frac{1}{\vec{S}_1 \times \vec{a}_1 \cdot \vec{a}_2} + \right. \\
& \frac{4}{3} \hat{n} \times \vec{S}_1 \cdot \vec{a}_2 \hat{n} \cdot \vec{a}_1 - \hat{n} \times \vec{S}_1 \cdot \vec{a}_2 \hat{n} \cdot \vec{a}_1 - \frac{4}{3} \hat{n} \times \vec{S}_1 \cdot \vec{a}_1 \hat{n} \cdot \vec{a}_2 - \frac{1}{3} \hat{n} \times \vec{S}_1 \cdot \vec{v}_1 \hat{n} \cdot \vec{a}_2 - \hat{n} \times \vec{S}_1 \cdot \vec{a}_1 \hat{n} \cdot \vec{a}_2 - \\
& \left. \hat{n} \times \vec{S}_1 \cdot \vec{a}_2 \hat{n} \cdot \vec{v}_1 + \frac{4}{3} \hat{n} \times \vec{S}_1 \cdot \vec{a}_2 \hat{n} \cdot \vec{v}_1 - \frac{8}{3} \frac{2}{\vec{S}_1 \times \vec{v}_1 \cdot \vec{a}_2} \log\left(\frac{r}{R_\theta}\right) + \frac{\frac{4}{3} \frac{1}{\vec{S}_1 \times \vec{a}_1 \cdot \vec{a}_2} + \frac{4}{3} \frac{2}{\vec{S}_1 \times \vec{v}_1 \cdot \vec{a}_2}}{\epsilon_d} \right) G^2 \Big\}
\end{aligned}$$

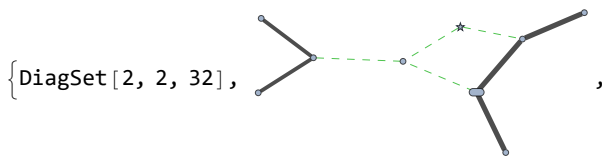

$$\begin{aligned}
& \frac{1}{r} \left( 4 \hat{n} \times \vec{S}_1 \cdot \vec{v}_2 (\hat{n} \cdot \vec{a}_1)^2 - \vec{S}_1 \times \vec{v}_1 \cdot \vec{v}_2 \hat{n} \cdot \vec{a}_1 + 3 \vec{S}_1 \times \vec{a}_1 \cdot \vec{v}_2 \hat{n} \cdot \vec{a}_1 - 2 \vec{S}_1 \times \vec{v}_1 \cdot \vec{a}_2 \hat{n} \cdot \vec{a}_1 + 2 \vec{S}_1 \times \vec{v}_2 \cdot \vec{a}_2 \hat{n} \cdot \vec{a}_1 + \right. \\
& \hat{n} \times \vec{S}_1 \cdot \vec{v}_1 \hat{n} \cdot \vec{a}_2 \hat{n} \cdot \vec{a}_1 + 4 \hat{n} \times \vec{S}_1 \cdot \vec{v}_2 \hat{n} \cdot \vec{a}_2 \hat{n} \cdot \vec{a}_1 + 8 \hat{n} \times \vec{S}_1 \cdot \vec{v}_2 \hat{n} \cdot \vec{v}_1 \hat{n} \cdot \vec{a}_1 - \hat{n} \times \vec{S}_1 \cdot \vec{a}_2 \hat{n} \cdot \vec{v}_1 \hat{n} \cdot \vec{a}_1 + \\
& \hat{n} \times \vec{S}_1 \cdot \vec{v}_1 \hat{n} \cdot \vec{v}_2 \hat{n} \cdot \vec{a}_1 + \frac{4}{3} \hat{n} \times \vec{S}_1 \cdot \vec{v}_2 \hat{n} \cdot \vec{v}_2 \hat{n} \cdot \vec{a}_1 + \hat{n} \times \vec{S}_1 \cdot \vec{a}_1 \hat{n} \cdot \vec{v}_2 \hat{n} \cdot \vec{a}_1 + 8 \hat{n} \times \vec{S}_1 \cdot \vec{a}_2 \hat{n} \cdot \vec{v}_2 \hat{n} \cdot \vec{a}_1 - \\
& \frac{1}{3} \hat{n} \times \vec{S}_1 \cdot \vec{a}_2 (\hat{n} \cdot \vec{v}_1)^2 - \frac{4}{3} \hat{n} \times \vec{S}_1 \cdot \vec{v}_2 (\hat{n} \cdot \vec{v}_1)^2 + \hat{n} \times \vec{S}_1 \cdot \vec{a}_2 (\hat{n} \cdot \vec{v}_1)^2 - \frac{4}{3} \hat{n} \times \vec{S}_1 \cdot \vec{a}_1 (\hat{n} \cdot \vec{v}_2)^2 + 4 \hat{n} \times \vec{S}_1 \cdot \vec{a}_1 (\hat{n} \cdot \vec{v}_2)^2 + \\
& 4 \vec{S}_1 \times \vec{a}_1 \cdot \vec{v}_2 \hat{n} \cdot \vec{v}_1 + \vec{S}_1 \times \vec{v}_1 \cdot \vec{a}_2 \hat{n} \cdot \vec{v}_1 + \vec{S}_1 \times \vec{v}_1 \cdot \vec{v}_2 \hat{n} \cdot \vec{v}_1 + \vec{S}_1 \times \vec{a}_1 \cdot \vec{v}_2 \hat{n} \cdot \vec{v}_1 + \frac{1}{3} \hat{n} \times \vec{S}_1 \cdot \vec{v}_1 \hat{n} \cdot \vec{a}_2 \hat{n} \cdot \vec{v}_1 + \\
& 3 \hat{n} \times \vec{S}_1 \cdot \vec{a}_1 \hat{n} \cdot \vec{a}_2 \hat{n} \cdot \vec{v}_1 - 2 \vec{S}_1 \times \vec{a}_1 \cdot \vec{v}_2 \hat{n} \cdot \vec{v}_2 + \vec{S}_1 \times \vec{v}_1 \cdot \vec{a}_1 \hat{n} \cdot \vec{v}_2 - 2 \vec{S}_1 \times \vec{a}_1 \cdot \vec{v}_2 \hat{n} \cdot \vec{v}_2 - \vec{S}_1 \times \vec{v}_1 \cdot \vec{a}_1 \hat{n} \cdot \vec{v}_2 + \\
& 4 \hat{n} \times \vec{S}_1 \cdot \vec{a}_1 \hat{n} \cdot \vec{v}_1 \hat{n} \cdot \vec{v}_2 + \frac{1}{3} \hat{n} \times \vec{S}_1 \cdot \vec{v}_1 \hat{n} \cdot \vec{v}_1 \hat{n} \cdot \vec{v}_2 - 5 \hat{n} \times \vec{S}_1 \cdot \vec{a}_1 \hat{n} \cdot \vec{v}_1 \hat{n} \cdot \vec{v}_2 - 2 \hat{n} \times \vec{S}_1 \cdot \vec{v}_1 \vec{a}_1 \cdot \vec{v}_2 - \\
& 2 \hat{n} \times \vec{S}_1 \cdot \vec{v}_2 \vec{a}_1 \cdot \vec{a}_1 + 7 \hat{n} \times \vec{S}_1 \cdot \vec{v}_1 \vec{a}_1 \cdot \vec{a}_2 - 2 \hat{n} \times \vec{S}_1 \cdot \vec{v}_2 \vec{a}_1 \cdot \vec{a}_2 + 5 \hat{n} \times \vec{S}_1 \cdot \vec{v}_1 \vec{a}_1 \cdot \vec{v}_2 - \frac{2}{3} \hat{n} \times \vec{S}_1 \cdot \vec{v}_2 \vec{a}_1 \cdot \vec{v}_2 + \\
& \hat{n} \times \vec{S}_1 \cdot \vec{a}_1 \vec{a}_1 \cdot \vec{v}_2 - 4 \hat{n} \times \vec{S}_1 \cdot \vec{a}_2 \vec{a}_1 \cdot \vec{v}_2 - 2 \hat{n} \times \vec{S}_1 \cdot \vec{v}_1 \vec{v}_1 \cdot \vec{a}_2 - 4 \hat{n} \times \vec{S}_1 \cdot \vec{v}_2 \vec{v}_1 \cdot \vec{a}_1 - \hat{n} \times \vec{S}_1 \cdot \vec{a}_2 \vec{v}_1 \cdot \vec{a}_1 - \\
& \frac{11}{3} \hat{n} \times \vec{S}_1 \cdot \vec{v}_1 \vec{v}_1 \cdot \vec{a}_2 + 5 \hat{n} \times \vec{S}_1 \cdot \vec{a}_1 \vec{v}_1 \cdot \vec{a}_2 + \frac{5}{3} \hat{n} \times \vec{S}_1 \cdot \vec{a}_2 \vec{v}_1 \cdot \vec{v}_1 + \frac{2}{3} \hat{n} \times \vec{S}_1 \cdot \vec{v}_2 \vec{v}_1 \cdot \vec{v}_1 + \hat{n} \times \vec{S}_1 \cdot \vec{a}_2 \vec{v}_1 \cdot \vec{v}_1 + \\
& 6 \hat{n} \times \vec{S}_1 \cdot \vec{a}_1 \vec{v}_1 \cdot \vec{v}_2 - \frac{5}{3} \hat{n} \times \vec{S}_1 \cdot \vec{v}_1 \vec{v}_1 \cdot \vec{v}_2 + \hat{n} \times \vec{S}_1 \cdot \vec{a}_1 \vec{v}_1 \cdot \vec{v}_2 + \frac{2}{3} \hat{n} \times \vec{S}_1 \cdot \vec{a}_1 \vec{v}_2 \cdot \vec{v}_2 - 2 \hat{n} \times \vec{S}_1 \cdot \vec{a}_1 \vec{v}_2 \cdot \vec{v}_2 \Big) m_1 m_2 G^2 + \\
& \frac{1}{r^2} \left( 8 \hat{n} \times \vec{S}_1 \cdot \vec{v}_2 (\hat{n} \cdot \vec{v}_1)^3 + \frac{2}{3} \hat{n} \times \vec{S}_1 \cdot \vec{a}_2 (\hat{n} \cdot \vec{v}_1)^3 + 2 \vec{S}_1 \times \vec{v}_1 \cdot \vec{v}_2 (\hat{n} \cdot \vec{v}_1)^2 - 2 \vec{S}_1 \times \vec{a}_1 \cdot \vec{v}_2 (\hat{n} \cdot \vec{v}_1)^2 + \right. \\
& \frac{1}{3} \vec{S}_1 \times \vec{v}_1 \cdot \vec{a}_2 (\hat{n} \cdot \vec{v}_1)^2 + \vec{S}_1 \times \vec{v}_2 \cdot \vec{a}_2 (\hat{n} \cdot \vec{v}_1)^2 - 16 \hat{n} \times \vec{S}_1 \cdot \vec{v}_2 \hat{n} \cdot \vec{a}_1 (\hat{n} \cdot \vec{v}_1)^2 - \frac{4}{3} \hat{n} \times \vec{S}_1 \cdot \vec{v}_1 \hat{n} \cdot \vec{a}_2 (\hat{n} \cdot \vec{v}_1)^2 + \\
& 4 \hat{n} \times \vec{S}_1 \cdot \vec{v}_2 \hat{n} \cdot \vec{a}_2 (\hat{n} \cdot \vec{v}_1)^2 - 2 \hat{n} \times \vec{S}_1 \cdot \vec{v}_1 \hat{n} \cdot \vec{v}_2 (\hat{n} \cdot \vec{v}_1)^2 - \frac{4}{3} \hat{n} \times \vec{S}_1 \cdot \vec{v}_2 \hat{n} \cdot \vec{v}_2 (\hat{n} \cdot \vec{v}_1)^2 - \\
& 10 \hat{n} \times \vec{S}_1 \cdot \vec{a}_1 \hat{n} \cdot \vec{v}_2 (\hat{n} \cdot \vec{v}_1)^2 + 8 \hat{n} \times \vec{S}_1 \cdot \vec{a}_2 \hat{n} \cdot \vec{v}_2 (\hat{n} \cdot \vec{v}_1)^2 + \frac{4}{3} \hat{n} \times \vec{S}_1 \cdot \vec{v}_1 (\hat{n} \cdot \vec{v}_2)^2 \hat{n} \cdot \vec{v}_1 + \\
& 12 \hat{n} \times \vec{S}_1 \cdot \vec{a}_1 (\hat{n} \cdot \vec{v}_2)^2 \hat{n} \cdot \vec{v}_1 - 4 \vec{S}_1 \times \vec{v}_1 \cdot \vec{v}_2 \hat{n} \cdot \vec{a}_1 \hat{n} \cdot \vec{v}_1 + \frac{5}{3} \vec{S}_1 \times \vec{v}_1 \cdot \vec{v}_2 \hat{n} \cdot \vec{v}_2 \hat{n} \cdot \vec{v}_1 - 3 \vec{S}_1 \times \vec{a}_1 \cdot \vec{v}_2 \hat{n} \cdot \vec{v}_2 \hat{n} \cdot \vec{v}_1 - \\
& \left. 3 \vec{S}_1 \times \vec{v}_1 \cdot \vec{a}_1 \hat{n} \cdot \vec{v}_2 \hat{n} \cdot \vec{v}_1 - 4 \hat{n} \times \vec{S}_1 \cdot \vec{v}_1 \hat{n} \cdot \vec{a}_1 \hat{n} \cdot \vec{v}_2 \hat{n} \cdot \vec{v}_1 - 4 \hat{n} \times \vec{S}_1 \cdot \vec{v}_2 \hat{n} \cdot \vec{a}_1 \hat{n} \cdot \vec{v}_2 \hat{n} \cdot \vec{v}_1 - \right)
\end{aligned}$$

$$\begin{aligned}
& 6 \hat{n} \times \vec{S}_1 \cdot \vec{v}_1 \vec{a}_1 \cdot \vec{v}_2 \hat{n} \cdot \vec{v}_1 + \hat{n} \times \vec{S}_1 \cdot \vec{v}_2 \vec{a}_1 \cdot \vec{v}_2 \hat{n} \cdot \vec{v}_1 + 11 \hat{n} \times \vec{S}_1 \cdot \vec{v}_2 \vec{v}_1 \cdot \vec{a}_1 \hat{n} \cdot \vec{v}_1 + \frac{5}{3} \hat{n} \times \vec{S}_1 \cdot \vec{v}_1 \vec{v}_1 \cdot \vec{a}_2 \hat{n} \cdot \vec{v}_1 - \\
& 2 \hat{n} \times \vec{S}_1 \cdot \vec{v}_2 \vec{v}_1 \cdot \vec{a}_2 \hat{n} \cdot \vec{v}_1 - 2 \hat{n} \times \vec{S}_1 \cdot \vec{a}_2 \vec{v}_1 \cdot \vec{v}_1 \hat{n} \cdot \vec{v}_1 + 2 \hat{n} \times \vec{S}_1 \cdot \vec{v}_1 \vec{v}_1 \cdot \vec{v}_2 \hat{n} \cdot \vec{v}_1 + \frac{2}{3} \hat{n} \times \vec{S}_1 \cdot \vec{v}_2 \vec{v}_1 \cdot \vec{v}_2 \hat{n} \cdot \vec{v}_1 - \\
& 7 \hat{n} \times \vec{S}_1 \cdot \vec{a}_1 \vec{v}_1 \cdot \vec{v}_2 \hat{n} \cdot \vec{v}_1 - 4 \hat{n} \times \vec{S}_1 \cdot \vec{a}_2 \vec{v}_1 \cdot \vec{v}_2 \hat{n} \cdot \vec{v}_1 - \frac{1}{3} \hat{n} \times \vec{S}_1 \cdot \vec{v}_1 \vec{v}_2 \cdot \vec{v}_2 \hat{n} \cdot \vec{v}_1 - 3 \hat{n} \times \vec{S}_1 \cdot \vec{a}_1 \vec{v}_2 \cdot \vec{v}_2 \hat{n} \cdot \vec{v}_1 + \\
& 4 \hat{n} \times \vec{S}_1 \cdot \vec{v}_1 \hat{n} \cdot \vec{a}_1 (\hat{n} \cdot \vec{v}_2)^2 + 16 \hat{n} \times \vec{S}_1 \cdot \vec{v}_2 \hat{n} \cdot \vec{a}_1 (\hat{n} \cdot \vec{v}_2)^2 - 5 \vec{S}_1 \times \vec{v}_1 \cdot \vec{v}_2 \hat{n} \cdot \vec{a}_1 \hat{n} \cdot \vec{v}_2 - 5 \vec{S}_1 \times \vec{v}_1 \cdot \vec{v}_2 \vec{a}_1 \cdot \vec{v}_2 + \\
& 13 \hat{n} \times \vec{S}_1 \cdot \vec{v}_1 \hat{n} \cdot \vec{v}_2 \vec{a}_1 \cdot \vec{v}_2 - 8 \hat{n} \times \vec{S}_1 \cdot \vec{v}_2 \hat{n} \cdot \vec{v}_2 \vec{a}_1 \cdot \vec{v}_2 + 5 \vec{S}_1 \times \vec{v}_1 \cdot \vec{v}_2 \vec{v}_1 \cdot \vec{a}_1 - 2 \hat{n} \times \vec{S}_1 \cdot \vec{v}_1 \hat{n} \cdot \vec{v}_2 \vec{v}_1 \cdot \vec{a}_1 - \\
& 2 \hat{n} \times \vec{S}_1 \cdot \vec{v}_2 \hat{n} \cdot \vec{v}_2 \vec{v}_1 \cdot \vec{a}_1 + 4 \vec{S}_1 \times \vec{v}_1 \cdot \vec{v}_2 \vec{v}_1 \cdot \vec{a}_2 - 8 \hat{n} \times \vec{S}_1 \cdot \vec{v}_1 \hat{n} \cdot \vec{v}_2 \vec{v}_1 \cdot \vec{a}_2 + 2 \vec{S}_1 \times \vec{v}_1 \cdot \vec{v}_2 \vec{v}_1 \cdot \vec{v}_1 + \\
& \vec{S}_1 \times \vec{a}_1 \cdot \vec{v}_2 \vec{v}_1 \cdot \vec{v}_1 - \frac{2}{3} \vec{S}_1 \times \vec{v}_1 \cdot \vec{a}_2 \vec{v}_1 \cdot \vec{v}_1 + \vec{S}_1 \times \vec{v}_2 \cdot \vec{a}_2 \vec{v}_1 \cdot \vec{v}_1 + \hat{n} \times \vec{S}_1 \cdot \vec{v}_2 \hat{n} \cdot \vec{a}_1 \vec{v}_1 \cdot \vec{v}_1 + \frac{7}{3} \hat{n} \times \vec{S}_1 \cdot \vec{v}_1 \hat{n} \cdot \vec{a}_2 \vec{v}_1 \cdot \vec{v}_1 + \\
& 2 \hat{n} \times \vec{S}_1 \cdot \vec{v}_2 \hat{n} \cdot \vec{a}_2 \vec{v}_1 \cdot \vec{v}_1 + 2 \hat{n} \times \vec{S}_1 \cdot \vec{v}_1 \hat{n} \cdot \vec{v}_2 \vec{v}_1 \cdot \vec{v}_1 + \frac{10}{3} \hat{n} \times \vec{S}_1 \cdot \vec{v}_2 \hat{n} \cdot \vec{v}_2 \vec{v}_1 \cdot \vec{v}_1 - 2 \hat{n} \times \vec{S}_1 \cdot \vec{a}_1 \hat{n} \cdot \vec{v}_2 \vec{v}_1 \cdot \vec{v}_1 + \\
& 4 \hat{n} \times \vec{S}_1 \cdot \vec{a}_2 \hat{n} \cdot \vec{v}_2 \vec{v}_1 \cdot \vec{v}_1 + \frac{8}{3} \vec{S}_1 \times \vec{v}_1 \cdot \vec{v}_2 \vec{v}_1 \cdot \vec{v}_2 - 5 \vec{S}_1 \times \vec{a}_1 \cdot \vec{v}_2 \vec{v}_1 \cdot \vec{v}_2 - 5 \vec{S}_1 \times \vec{v}_1 \cdot \vec{a}_1 \vec{v}_1 \cdot \vec{v}_2 + 2 \vec{S}_1 \times \vec{v}_1 \cdot \vec{a}_2 \vec{v}_1 \cdot \vec{v}_2 + \\
& 5 \hat{n} \times \vec{S}_1 \cdot \vec{v}_1 \hat{n} \cdot \vec{a}_1 \vec{v}_1 \cdot \vec{v}_2 + \hat{n} \times \vec{S}_1 \cdot \vec{v}_2 \hat{n} \cdot \vec{a}_1 \vec{v}_1 \cdot \vec{v}_2 - 4 \hat{n} \times \vec{S}_1 \cdot \vec{v}_1 \hat{n} \cdot \vec{a}_2 \vec{v}_1 \cdot \vec{v}_2 - \frac{23}{3} \hat{n} \times \vec{S}_1 \cdot \vec{v}_1 \hat{n} \cdot \vec{v}_2 \vec{v}_1 \cdot \vec{v}_2 + \\
& 7 \hat{n} \times \vec{S}_1 \cdot \vec{a}_1 \hat{n} \cdot \vec{v}_2 \vec{v}_1 \cdot \vec{v}_2 - \hat{n} \times \vec{S}_1 \cdot \vec{v}_1 \hat{n} \cdot \vec{a}_1 \vec{v}_2 \cdot \vec{v}_2 - 4 \hat{n} \times \vec{S}_1 \cdot \vec{v}_2 \hat{n} \cdot \vec{a}_1 \vec{v}_2 \cdot \vec{v}_2 \Big) m_1 m_2 G^2 + \frac{1}{r^3} \\
& \left( -20 \hat{n} \times \vec{S}_1 \cdot \vec{v}_2 (\hat{n} \cdot \vec{v}_1)^4 - \frac{23}{3} \vec{S}_1 \times \vec{v}_1 \cdot \vec{v}_2 (\hat{n} \cdot \vec{v}_1)^3 + 5 \hat{n} \times \vec{S}_1 \cdot \vec{v}_1 \hat{n} \cdot \vec{v}_2 (\hat{n} \cdot \vec{v}_1)^3 + 4 \hat{n} \times \vec{S}_1 \cdot \vec{v}_2 \hat{n} \cdot \vec{v}_2 (\hat{n} \cdot \vec{v}_1)^3 - \right. \\
& 8 \hat{n} \times \vec{S}_1 \cdot \vec{v}_1 (\hat{n} \cdot \vec{v}_2)^2 (\hat{n} \cdot \vec{v}_1)^2 + 24 \hat{n} \times \vec{S}_1 \cdot \vec{v}_2 (\hat{n} \cdot \vec{v}_2)^2 (\hat{n} \cdot \vec{v}_1)^2 + \frac{8}{3} \vec{S}_1 \times \vec{v}_1 \cdot \vec{v}_2 \hat{n} \cdot \vec{v}_2 (\hat{n} \cdot \vec{v}_1)^2 + \\
& 2 \hat{n} \times \vec{S}_1 \cdot \vec{v}_2 \vec{v}_1 \cdot \vec{v}_1 (\hat{n} \cdot \vec{v}_1)^2 - 5 \hat{n} \times \vec{S}_1 \cdot \vec{v}_1 \vec{v}_1 \cdot \vec{v}_2 (\hat{n} \cdot \vec{v}_1)^2 - 2 \hat{n} \times \vec{S}_1 \cdot \vec{v}_2 \vec{v}_1 \cdot \vec{v}_2 (\hat{n} \cdot \vec{v}_1)^2 + \\
& \frac{4}{3} \hat{n} \times \vec{S}_1 \cdot \vec{v}_1 \vec{v}_2 \cdot \vec{v}_2 (\hat{n} \cdot \vec{v}_1)^2 - 4 \hat{n} \times \vec{S}_1 \cdot \vec{v}_2 \vec{v}_2 \cdot \vec{v}_2 (\hat{n} \cdot \vec{v}_1)^2 - \vec{S}_1 \times \vec{v}_1 \cdot \vec{v}_2 \vec{v}_1 \cdot \vec{v}_1 \hat{n} \cdot \vec{v}_1 - \\
& 7 \hat{n} \times \vec{S}_1 \cdot \vec{v}_1 \hat{n} \cdot \vec{v}_2 \vec{v}_1 \cdot \vec{v}_1 \hat{n} \cdot \vec{v}_1 - 8 \hat{n} \times \vec{S}_1 \cdot \vec{v}_2 \hat{n} \cdot \vec{v}_2 \vec{v}_1 \cdot \vec{v}_1 \hat{n} \cdot \vec{v}_1 - \frac{7}{3} \vec{S}_1 \times \vec{v}_1 \cdot \vec{v}_2 \vec{v}_1 \cdot \vec{v}_2 \hat{n} \cdot \vec{v}_1 + \\
& \frac{28}{3} \hat{n} \times \vec{S}_1 \cdot \vec{v}_1 \hat{n} \cdot \vec{v}_2 \vec{v}_1 \cdot \vec{v}_2 \hat{n} \cdot \vec{v}_1 - 16 \hat{n} \times \vec{S}_1 \cdot \vec{v}_2 \hat{n} \cdot \vec{v}_2 \vec{v}_1 \cdot \vec{v}_2 \hat{n} \cdot \vec{v}_1 + 2 \hat{n} \times \vec{S}_1 \cdot \vec{v}_2 (\vec{v}_1 \cdot \vec{v}_1)^2 - \frac{5}{3} \hat{n} \times \vec{S}_1 \cdot \vec{v}_1 (\vec{v}_1 \cdot \vec{v}_2)^2 + \\
& 2 \hat{n} \times \vec{S}_1 \cdot \vec{v}_2 (\vec{v}_1 \cdot \vec{v}_2)^2 + \frac{28}{3} \hat{n} \times \vec{S}_1 \cdot \vec{v}_1 (\hat{n} \cdot \vec{v}_2)^2 \vec{v}_1 \cdot \vec{v}_1 + 8 \hat{n} \times \vec{S}_1 \cdot \vec{v}_2 (\hat{n} \cdot \vec{v}_2)^2 \vec{v}_1 \cdot \vec{v}_1 - \frac{11}{3} \vec{S}_1 \times \vec{v}_1 \cdot \vec{v}_2 \hat{n} \cdot \vec{v}_2 \vec{v}_1 \cdot \vec{v}_1 - \\
& 16 \hat{n} \times \vec{S}_1 \cdot \vec{v}_1 (\hat{n} \cdot \vec{v}_2)^2 \vec{v}_1 \cdot \vec{v}_2 + 8 \vec{S}_1 \times \vec{v}_1 \cdot \vec{v}_2 \hat{n} \cdot \vec{v}_2 \vec{v}_1 \cdot \vec{v}_2 - \hat{n} \times \vec{S}_1 \cdot \vec{v}_1 \vec{v}_1 \cdot \vec{v}_1 \vec{v}_1 \cdot \vec{v}_2 + 2 \hat{n} \times \vec{S}_1 \cdot \vec{v}_2 \vec{v}_1 \cdot \vec{v}_1 \vec{v}_1 \cdot \vec{v}_2 - \\
& \left. \frac{7}{3} \hat{n} \times \vec{S}_1 \cdot \vec{v}_1 \vec{v}_1 \cdot \vec{v}_1 \vec{v}_2 \cdot \vec{v}_2 - 2 \hat{n} \times \vec{S}_1 \cdot \vec{v}_2 \vec{v}_1 \cdot \vec{v}_1 \vec{v}_2 \cdot \vec{v}_2 + 4 \hat{n} \times \vec{S}_1 \cdot \vec{v}_1 \vec{v}_1 \cdot \vec{v}_2 \vec{v}_2 \cdot \vec{v}_2 \right) m_1 m_2 G^2 + \\
& m_1 m_2 \left( -\frac{2}{3} \vec{S}_1 \times \vec{a}_1 \cdot \vec{v}_2 - \frac{16}{9} \vec{S}_1 \times \vec{a}_1 \cdot \vec{a}_2 - \frac{22}{9} \vec{S}_1 \times \vec{a}_1 \cdot \vec{v}_2 - \frac{2}{3} \vec{S}_1 \times \vec{a}_1 \cdot \vec{a}_2 + \frac{2}{3} \vec{S}_1 \times \vec{a}_1 \cdot \vec{a}_2 + \frac{2}{3} \hat{n} \times \vec{S}_1 \cdot \vec{a}_2 \hat{n} \cdot \vec{a}_1 - \right. \\
& \frac{4}{3} \hat{n} \times \vec{S}_1 \cdot \vec{v}_2 \hat{n} \cdot \vec{a}_1 + 2 \hat{n} \times \vec{S}_1 \cdot \vec{a}_2 \hat{n} \cdot \vec{a}_1 - \frac{2}{3} \hat{n} \times \vec{S}_1 \cdot \vec{a}_1 \hat{n} \cdot \vec{a}_2 + 2 \hat{n} \times \vec{S}_1 \cdot \vec{a}_1 \hat{n} \cdot \vec{a}_2 + 2 \hat{n} \times \vec{S}_1 \cdot \vec{a}_1 \hat{n} \cdot \vec{v}_2 - \\
& \left. \frac{2}{3} \hat{n} \times \vec{S}_1 \cdot \vec{a}_1 \hat{n} \cdot \vec{v}_2 + \frac{8}{3} \vec{S}_1 \times \vec{a}_1 \cdot \vec{a}_2 \log\left(\frac{r}{R_\theta}\right) + \frac{8}{3} \vec{S}_1 \times \vec{a}_1 \cdot \vec{v}_2 \log\left(\frac{r}{R_\theta}\right) + \frac{-\frac{4}{3} \vec{S}_1 \times \vec{a}_1 \cdot \vec{a}_2 - \frac{4}{3} \vec{S}_1 \times \vec{a}_1 \cdot \vec{v}_2}{\epsilon_d} \right) G^2 \Big\}
\end{aligned}$$

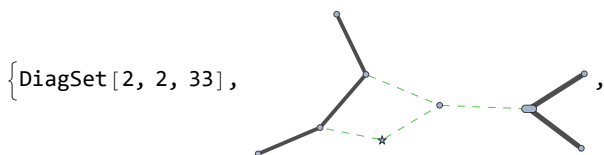

$$\frac{1}{r} G^2 \left( \frac{8}{3} \hat{n} \times \vec{S}_1 \cdot \vec{v}_2 (\hat{n} \cdot \vec{v}_2)^2 + \frac{16}{3} \hat{n} \times \vec{a}_2 \cdot \vec{S}_1 (\hat{n} \cdot \vec{v}_2)^2 - \frac{4}{3} \vec{a}_1 \times \vec{a}_2 \cdot \vec{S}_1 \hat{n} \cdot \vec{v}_2 - \frac{8}{3} \vec{a}_2 \times \vec{S}_1 \cdot \vec{v}_1 \hat{n} \cdot \vec{v}_2 - \right.$$

$$\begin{aligned}
& 4 \vec{a}_2 \times \vec{S}_1 \cdot \vec{v}_2 \hat{n} \cdot \vec{v}_2 + \frac{8}{3} \hat{n} \times \vec{a}_2 \cdot \vec{S}_1 \hat{n} \cdot \vec{a}_1 \hat{n} \cdot \vec{v}_2 - \frac{8}{3} \hat{n} \times \vec{S}_1 \cdot \vec{v}_2 \hat{n} \cdot \vec{a}_2 \hat{n} \cdot \vec{v}_2 + \frac{16}{3} \hat{n} \times \vec{a}_2 \cdot \vec{S}_1 \hat{n} \cdot \vec{v}_1 \hat{n} \cdot \vec{v}_2 - \\
& \frac{8}{3} \vec{a}_2 \times \vec{S}_1 \cdot \vec{v}_2 \hat{n} \cdot \vec{a}_1 + \frac{8}{3} \vec{S}_1 \times \vec{v}_1 \cdot \vec{v}_2 \hat{n} \cdot \vec{a}_2 - \frac{4}{3} \vec{a}_1 \times \vec{S}_1 \cdot \vec{v}_2 \hat{n} \cdot \vec{a}_2 + \frac{8}{3} \hat{n} \times \vec{S}_1 \cdot \vec{v}_2 \hat{n} \cdot \vec{a}_1 \hat{n} \cdot \vec{a}_2 - \\
& \frac{16}{3} \vec{a}_2 \times \vec{S}_1 \cdot \vec{v}_2 \hat{n} \cdot \vec{v}_1 + \frac{16}{3} \hat{n} \times \vec{S}_1 \cdot \vec{v}_2 \hat{n} \cdot \vec{a}_2 \hat{n} \cdot \vec{v}_1 - 4 \hat{n} \times \vec{S}_1 \cdot \vec{v}_2 \vec{a}_2 \cdot \vec{v}_2 - \frac{4}{3} \hat{n} \times \vec{S}_1 \cdot \vec{v}_2 \vec{a}_1 \cdot \vec{a}_2 - \\
& \frac{4}{3} \hat{n} \times \vec{a}_2 \cdot \vec{S}_1 \vec{a}_1 \cdot \vec{v}_2 + 8 \hat{n} \times \vec{S}_1 \cdot \vec{v}_2 \vec{a}_2 \cdot \vec{a}_2 - \frac{8}{3} \hat{n} \times \vec{S}_1 \cdot \vec{v}_2 \vec{a}_2 \cdot \vec{v}_1 + \frac{4}{3} \hat{n} \times \vec{S}_1 \cdot \vec{v}_2 \vec{a}_2 \cdot \vec{v}_2 - \\
& 4 \hat{n} \times \vec{a}_2 \cdot \vec{S}_1 \vec{a}_2 \cdot \vec{v}_2 - \frac{8}{3} \hat{n} \times \vec{a}_2 \cdot \vec{S}_1 \vec{v}_1 \cdot \vec{v}_2 - \frac{4}{3} \hat{n} \times \vec{S}_1 \cdot \vec{v}_2 \vec{v}_2 \cdot \vec{v}_2 - \frac{26}{3} \hat{n} \times \vec{a}_2 \cdot \vec{S}_1 \vec{v}_2 \cdot \vec{v}_2 \Big) m_2^2 + \frac{1}{r^2} \\
& G^2 \left( -\frac{16}{3} \hat{n} \times \vec{S}_1 \cdot \vec{v}_2 (\hat{n} \cdot \vec{v}_2)^3 + \frac{64}{3} \hat{n} \times \vec{a}_2 \cdot \vec{S}_1 (\hat{n} \cdot \vec{v}_2)^3 - \frac{16}{3} \vec{S}_1 \times \vec{v}_1 \cdot \vec{v}_2 (\hat{n} \cdot \vec{v}_2)^2 + \frac{8}{3} \vec{a}_1 \times \vec{S}_1 \cdot \vec{v}_2 (\hat{n} \cdot \vec{v}_2)^2 + \right. \\
& \frac{16}{3} \vec{a}_2 \times \vec{S}_1 \cdot \vec{v}_1 (\hat{n} \cdot \vec{v}_2)^2 - 16 \vec{a}_2 \times \vec{S}_1 \cdot \vec{v}_2 (\hat{n} \cdot \vec{v}_2)^2 - \frac{32}{3} \hat{n} \times \vec{S}_1 \cdot \vec{v}_2 \hat{n} \cdot \vec{a}_1 (\hat{n} \cdot \vec{v}_2)^2 - \frac{64}{3} \hat{n} \times \vec{S}_1 \cdot \vec{v}_2 \hat{n} \cdot \vec{v}_1 (\hat{n} \cdot \vec{v}_2)^2 - \\
& \frac{64}{3} \hat{n} \times \vec{a}_2 \cdot \vec{S}_1 \hat{n} \cdot \vec{v}_1 (\hat{n} \cdot \vec{v}_2)^2 - \frac{32}{3} \hat{n} \times \vec{a}_2 \cdot \vec{S}_1 (\hat{n} \cdot \vec{v}_1)^2 \hat{n} \cdot \vec{v}_2 + \frac{8}{3} \vec{S}_1 \times \vec{v}_1 \cdot \vec{v}_2 \hat{n} \cdot \vec{a}_2 \hat{n} \cdot \vec{v}_2 + \\
& \frac{16}{3} \vec{a}_2 \times \vec{S}_1 \cdot \vec{v}_1 \hat{n} \cdot \vec{v}_1 \hat{n} \cdot \vec{v}_2 + 8 \vec{a}_2 \times \vec{S}_1 \cdot \vec{v}_2 \hat{n} \cdot \vec{v}_1 \hat{n} \cdot \vec{v}_2 + \frac{32}{3} \hat{n} \times \vec{S}_1 \cdot \vec{v}_2 \hat{n} \cdot \vec{a}_2 \hat{n} \cdot \vec{v}_1 \hat{n} \cdot \vec{v}_2 + \\
& \frac{16}{3} \hat{n} \times \vec{S}_1 \cdot \vec{v}_2 \vec{a}_1 \cdot \vec{v}_2 \hat{n} \cdot \vec{v}_2 - \frac{8}{3} \hat{n} \times \vec{S}_1 \cdot \vec{v}_2 \vec{a}_2 \cdot \vec{v}_1 \hat{n} \cdot \vec{v}_2 + \frac{8}{3} \hat{n} \times \vec{a}_2 \cdot \vec{S}_1 \vec{v}_1 \cdot \vec{v}_1 \hat{n} \cdot \vec{v}_2 + \frac{32}{3} \hat{n} \times \vec{S}_1 \cdot \vec{v}_2 \vec{v}_1 \cdot \vec{v}_2 \hat{n} \cdot \vec{v}_2 + \\
& \frac{32}{3} \hat{n} \times \vec{a}_2 \cdot \vec{S}_1 \vec{v}_1 \cdot \vec{v}_2 \hat{n} \cdot \vec{v}_2 + 8 \hat{n} \times \vec{S}_1 \cdot \vec{v}_2 \vec{v}_2 \cdot \vec{v}_2 \hat{n} \cdot \vec{v}_2 - 4 \hat{n} \times \vec{a}_2 \cdot \vec{S}_1 \vec{v}_2 \cdot \vec{v}_2 \hat{n} \cdot \vec{v}_2 + \frac{16}{3} \vec{a}_2 \times \vec{S}_1 \cdot \vec{v}_2 (\hat{n} \cdot \vec{v}_1)^2 - \\
& \frac{32}{3} \hat{n} \times \vec{S}_1 \cdot \vec{v}_2 \hat{n} \cdot \vec{a}_2 (\hat{n} \cdot \vec{v}_1)^2 - \frac{16}{3} \vec{S}_1 \times \vec{v}_1 \cdot \vec{v}_2 \hat{n} \cdot \vec{a}_2 \hat{n} \cdot \vec{v}_1 + \frac{8}{3} \vec{S}_1 \times \vec{v}_1 \cdot \vec{v}_2 \vec{a}_2 \cdot \vec{v}_1 + \frac{16}{3} \hat{n} \times \vec{S}_1 \cdot \vec{v}_2 \hat{n} \cdot \vec{v}_1 \vec{a}_2 \cdot \vec{v}_1 - \\
& \frac{4}{3} \vec{S}_1 \times \vec{v}_1 \cdot \vec{v}_2 \vec{a}_2 \cdot \vec{v}_2 - \frac{8}{3} \hat{n} \times \vec{S}_1 \cdot \vec{v}_2 \hat{n} \cdot \vec{v}_1 \vec{a}_2 \cdot \vec{v}_2 - \frac{8}{3} \vec{a}_2 \times \vec{S}_1 \cdot \vec{v}_2 \vec{v}_1 \cdot \vec{v}_1 + \frac{8}{3} \hat{n} \times \vec{S}_1 \cdot \vec{v}_2 \hat{n} \cdot \vec{a}_2 \vec{v}_1 \cdot \vec{v}_1 - \\
& \frac{8}{3} \vec{a}_2 \times \vec{S}_1 \cdot \vec{v}_1 \vec{v}_1 \cdot \vec{v}_2 - 4 \vec{a}_2 \times \vec{S}_1 \cdot \vec{v}_2 \vec{v}_1 \cdot \vec{v}_2 - \frac{8}{3} \hat{n} \times \vec{S}_1 \cdot \vec{v}_2 \hat{n} \cdot \vec{a}_2 \vec{v}_1 \cdot \vec{v}_2 + \frac{16}{3} \hat{n} \times \vec{a}_2 \cdot \vec{S}_1 \hat{n} \cdot \vec{v}_1 \vec{v}_1 \cdot \vec{v}_2 + \\
& \frac{8}{3} \vec{S}_1 \times \vec{v}_1 \cdot \vec{v}_2 \vec{v}_2 \cdot \vec{v}_2 - \frac{4}{3} \vec{a}_1 \times \vec{S}_1 \cdot \vec{v}_2 \vec{v}_2 \cdot \vec{v}_2 - \frac{26}{3} \vec{a}_2 \times \vec{S}_1 \cdot \vec{v}_1 \vec{v}_2 \cdot \vec{v}_2 + \frac{8}{3} \hat{n} \times \vec{S}_1 \cdot \vec{v}_2 \hat{n} \cdot \vec{a}_1 \vec{v}_2 \cdot \vec{v}_2 + \\
& 4 \hat{n} \times \vec{S}_1 \cdot \vec{v}_2 \hat{n} \cdot \vec{a}_2 \vec{v}_2 \cdot \vec{v}_2 + \frac{16}{3} \hat{n} \times \vec{S}_1 \cdot \vec{v}_2 \hat{n} \cdot \vec{v}_1 \vec{v}_2 \cdot \vec{v}_2 + \frac{52}{3} \hat{n} \times \vec{a}_2 \cdot \vec{S}_1 \hat{n} \cdot \vec{v}_1 \vec{v}_2 \cdot \vec{v}_2 \Big) m_2^2 + \frac{1}{r^3} \\
& G^2 \left( -32 \hat{n} \times \vec{S}_1 \cdot \vec{v}_2 (\hat{n} \cdot \vec{v}_2)^4 + \frac{16}{3} \vec{S}_1 \times \vec{v}_1 \cdot \vec{v}_2 (\hat{n} \cdot \vec{v}_2)^3 + 32 \hat{n} \times \vec{S}_1 \cdot \vec{v}_2 \hat{n} \cdot \vec{v}_1 (\hat{n} \cdot \vec{v}_2)^3 + 64 \hat{n} \times \vec{S}_1 \cdot \vec{v}_2 (\hat{n} \cdot \vec{v}_1)^2 (\hat{n} \cdot \vec{v}_2)^2 + \right. \\
& \frac{64}{3} \vec{S}_1 \times \vec{v}_1 \cdot \vec{v}_2 \hat{n} \cdot \vec{v}_1 (\hat{n} \cdot \vec{v}_2)^2 - \frac{32}{3} \hat{n} \times \vec{S}_1 \cdot \vec{v}_2 \vec{v}_1 \cdot \vec{v}_1 (\hat{n} \cdot \vec{v}_2)^2 - 16 \hat{n} \times \vec{S}_1 \cdot \vec{v}_2 \vec{v}_1 \cdot \vec{v}_2 (\hat{n} \cdot \vec{v}_2)^2 + \\
& 12 \hat{n} \times \vec{S}_1 \cdot \vec{v}_2 \vec{v}_2 \cdot \vec{v}_2 (\hat{n} \cdot \vec{v}_2)^2 - \frac{32}{3} \vec{S}_1 \times \vec{v}_1 \cdot \vec{v}_2 \vec{v}_1 \cdot \vec{v}_2 \hat{n} \cdot \vec{v}_2 - \frac{128}{3} \hat{n} \times \vec{S}_1 \cdot \vec{v}_2 \hat{n} \cdot \vec{v}_1 \vec{v}_1 \cdot \vec{v}_2 \hat{n} \cdot \vec{v}_2 - \\
& 8 \vec{S}_1 \times \vec{v}_1 \cdot \vec{v}_2 \vec{v}_2 \cdot \vec{v}_2 \hat{n} \cdot \vec{v}_2 - 32 \hat{n} \times \vec{S}_1 \cdot \vec{v}_2 \hat{n} \cdot \vec{v}_1 \vec{v}_2 \cdot \vec{v}_2 \hat{n} \cdot \vec{v}_2 + \frac{16}{3} \hat{n} \times \vec{S}_1 \cdot \vec{v}_2 (\vec{v}_1 \cdot \vec{v}_2)^2 - 2 \hat{n} \times \vec{S}_1 \cdot \vec{v}_2 (\vec{v}_2 \cdot \vec{v}_2)^2 - \\
& \left. \frac{32}{3} \hat{n} \times \vec{S}_1 \cdot \vec{v}_2 (\hat{n} \cdot \vec{v}_1)^2 \vec{v}_2 \cdot \vec{v}_2 - \frac{16}{3} \vec{S}_1 \times \vec{v}_1 \cdot \vec{v}_2 \hat{n} \cdot \vec{v}_1 \vec{v}_2 \cdot \vec{v}_2 + \frac{8}{3} \hat{n} \times \vec{S}_1 \cdot \vec{v}_2 \vec{v}_1 \cdot \vec{v}_1 \vec{v}_2 \cdot \vec{v}_2 + 8 \hat{n} \times \vec{S}_1 \cdot \vec{v}_2 \vec{v}_1 \cdot \vec{v}_2 \vec{v}_2 \cdot \vec{v}_2 \right) \\
& m_2^2 + G^2 \left( \frac{4}{3} \vec{a}_2 \times \vec{S}_1 \cdot \vec{v}_2 + \frac{8}{3} \vec{a}_2 \times \vec{a}_2 \cdot \vec{S}_1 + \frac{16}{9} \vec{a}_2 \times \vec{S}_1 \cdot \vec{v}_2 - \frac{4}{3} \hat{n} \times \vec{S}_1 \cdot \vec{v}_2 \hat{n} \cdot \vec{a}_2 - \right. \\
& \left. \frac{4}{3} \hat{n} \times \vec{a}_2 \cdot \vec{S}_1 \hat{n} \cdot \vec{v}_2 - \frac{8}{3} \vec{a}_2 \times \vec{S}_1 \cdot \vec{v}_2 \log \left( \frac{r}{R_0} \right) + \frac{4 \vec{a}_2 \times \vec{S}_1 \cdot \vec{v}_2}{3 \in_d} \right) m_2^2 \Big\}
\end{aligned}$$

{DiagSet[2, 2, 34],

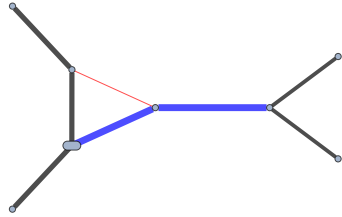

,

$$\begin{aligned} & \frac{1}{r^2} G^2 m_1 m_2 \left( 8 \vec{a}_1 \cdot \vec{v}_2 \hat{n} \cdot \vec{v}_2 \hat{n} \times \vec{S}_1 \cdot \vec{v}_2 - 6 \vec{v}_1 \cdot \vec{a}_2 \hat{n} \cdot \vec{v}_1 \hat{n} \times \vec{S}_1 \cdot \vec{v}_2 - 6 \vec{v}_1 \cdot \vec{v}_2 \hat{n} \cdot \vec{v}_1 \hat{n} \times \vec{S}_1 \cdot \vec{a}_2 + \right. \\ & 12 \vec{v}_2 \cdot \vec{a}_2 \hat{n} \cdot \vec{v}_1 \hat{n} \times \vec{S}_1 \cdot \vec{v}_1 - 8 \vec{v}_2 \cdot \vec{v}_2 \hat{n} \cdot \vec{v}_2 \hat{n} \times \vec{S}_1 \cdot \vec{a}_1 - 2 \vec{v}_1 \cdot \vec{a}_2 \vec{S}_1 \times \vec{v}_1 \cdot \vec{v}_2 - 2 \vec{v}_1 \cdot \vec{v}_2 \vec{S}_1 \times \vec{v}_1 \cdot \vec{a}_2 + \\ & \left. 4 \vec{v}_2 \cdot \vec{v}_2 \vec{S}_1 \times \vec{a}_1 \cdot \vec{v}_2 + 8 \vec{v}_1 \cdot \vec{v}_2 \hat{n} \cdot \vec{v}_2 \hat{n} \times \vec{S}_1 \cdot \vec{v}_2 - 8 \vec{v}_2 \cdot \vec{v}_2 \hat{n} \cdot \vec{v}_2 \hat{n} \times \vec{S}_1 \cdot \vec{v}_1 + 4 \vec{v}_2 \cdot \vec{v}_2 \vec{S}_1 \times \vec{v}_1 \cdot \vec{v}_2 \right) + \\ & \frac{1}{r} G^2 m_1 m_2 \left( 4 \vec{a}_1 \cdot \vec{a}_2 \hat{n} \times \vec{S}_1 \cdot \vec{v}_2 + 4 \vec{a}_1 \cdot \vec{v}_2 \hat{n} \times \vec{S}_1 \cdot \vec{a}_2 + 4 \vec{v}_1 \cdot \vec{a}_2 \hat{n} \times \vec{S}_1 \cdot \vec{v}_2 + 4 \vec{v}_1 \cdot \vec{v}_2 \hat{n} \times \vec{S}_1 \cdot \vec{a}_2 - \right. \\ & \left. 8 \vec{v}_2 \cdot \vec{a}_2 \hat{n} \times \vec{S}_1 \cdot \vec{v}_1 - 8 \vec{v}_2 \cdot \vec{a}_2 \hat{n} \times \vec{S}_1 \cdot \vec{a}_1 \right) + \frac{1}{r^3} \\ & G^2 m_1 m_2 \left( 6 (\vec{v}_1 \cdot \vec{v}_2)^2 \hat{n} \times \vec{S}_1 \cdot \vec{v}_2 - 4 \vec{v}_1 \cdot \vec{v}_2 \hat{n} \cdot \vec{v}_2 \vec{S}_1 \times \vec{v}_1 \cdot \vec{v}_2 - 24 \vec{v}_1 \cdot \vec{v}_2 \hat{n} \cdot \vec{v}_1 \hat{n} \cdot \vec{v}_2 \hat{n} \times \vec{S}_1 \cdot \vec{v}_2 - \right. \\ & \left. 6 \vec{v}_2 \cdot \vec{v}_2 \vec{v}_1 \cdot \vec{v}_2 \hat{n} \times \vec{S}_1 \cdot \vec{v}_1 - 6 \vec{v}_2 \cdot \vec{v}_2 \hat{n} \cdot \vec{v}_1 \vec{S}_1 \times \vec{v}_1 \cdot \vec{v}_2 + 24 \vec{v}_2 \cdot \vec{v}_2 \hat{n} \cdot \vec{v}_1 \hat{n} \cdot \vec{v}_2 \hat{n} \times \vec{S}_1 \cdot \vec{v}_1 \right) \} \end{aligned}$$

{DiagSet[2, 2, 35],

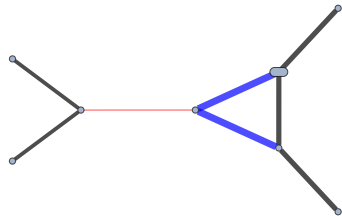

$$, \frac{G^2 m_1 m_2 \left( 4 \vec{v}_1 \cdot \vec{a}_1 \hat{n} \cdot \vec{v}_1 \hat{n} \times \vec{S}_1 \cdot \vec{v}_1 - 4 \vec{v}_1 \cdot \vec{v}_1 \hat{n} \cdot \vec{v}_1 \hat{n} \times \vec{S}_1 \cdot \vec{a}_1 \right)}{r^2} +$$

$$\frac{1}{r} G^2 m_1 m_2 \left( 4 \vec{a}_1 \cdot \vec{a}_1 \hat{n} \times \vec{S}_1 \cdot \vec{v}_1 - 4 \vec{v}_1 \cdot \vec{a}_1 \hat{n} \times \vec{S}_1 \cdot \vec{v}_1 - 4 \vec{v}_1 \cdot \vec{a}_1 \hat{n} \times \vec{S}_1 \cdot \vec{a}_1 + 4 \vec{v}_1 \cdot \vec{v}_1 \hat{n} \times \vec{S}_1 \cdot \vec{a}_1 \right) \}$$

{DiagSet[2, 2, 36],

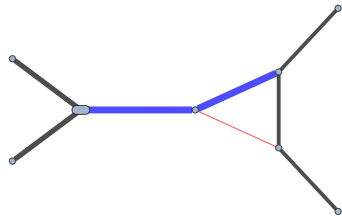

,

$$\begin{aligned} & \frac{1}{r^2} G^2 m_2^2 \left( 8 \vec{a}_1 \cdot \vec{v}_2 \hat{n} \cdot \vec{v}_2 \hat{n} \times \vec{S}_1 \cdot \vec{v}_2 - 16 \vec{a}_2 \cdot \vec{v}_1 \hat{n} \cdot \vec{v}_1 \hat{n} \times \vec{S}_1 \cdot \vec{v}_2 + 32 \vec{a}_2 \cdot \vec{v}_2 \hat{n} \cdot \vec{v}_1 \hat{n} \times \vec{S}_1 \cdot \vec{v}_1 + \right. \\ & 16 \vec{v}_1 \cdot \vec{v}_2 \hat{n} \cdot \vec{v}_1 \hat{n} \times \vec{a}_2 \cdot \vec{S}_1 + 8 \vec{v}_2 \cdot \vec{v}_2 \hat{n} \cdot \vec{v}_2 \hat{n} \times \vec{a}_1 \cdot \vec{S}_1 - 8 \vec{a}_2 \cdot \vec{v}_1 \vec{S}_1 \times \vec{v}_1 \cdot \vec{v}_2 - 8 \vec{v}_1 \cdot \vec{v}_2 \vec{a}_2 \times \vec{S}_1 \cdot \vec{v}_1 - \\ & \left. 4 \vec{v}_2 \cdot \vec{v}_2 \vec{a}_1 \times \vec{S}_1 \cdot \vec{v}_2 + 8 \vec{v}_1 \cdot \vec{v}_2 \hat{n} \cdot \vec{v}_2 \hat{n} \times \vec{S}_1 \cdot \vec{v}_2 - 8 \vec{v}_2 \cdot \vec{v}_2 \hat{n} \cdot \vec{v}_2 \hat{n} \times \vec{S}_1 \cdot \vec{v}_1 + 4 \vec{v}_2 \cdot \vec{v}_2 \vec{S}_1 \times \vec{v}_1 \cdot \vec{v}_2 \right) + \\ & \frac{1}{r} G^2 m_2^2 \left( 8 \vec{a}_1 \cdot \vec{a}_2 \hat{n} \times \vec{S}_1 \cdot \vec{v}_2 - 8 \vec{a}_1 \cdot \vec{v}_2 \hat{n} \times \vec{a}_2 \cdot \vec{S}_1 + 8 \vec{a}_2 \cdot \vec{v}_1 \hat{n} \times \vec{S}_1 \cdot \vec{v}_2 - 16 \vec{a}_2 \cdot \vec{v}_2 \hat{n} \times \vec{S}_1 \cdot \vec{v}_1 + \right. \\ & \left. 16 \vec{a}_2 \cdot \vec{v}_2 \hat{n} \times \vec{a}_1 \cdot \vec{S}_1 - 8 \vec{v}_1 \cdot \vec{v}_2 \hat{n} \times \vec{a}_2 \cdot \vec{S}_1 \right) + \frac{1}{r^3} \\ & G^2 m_2^2 \left( 8 (\vec{v}_1 \cdot \vec{v}_2)^2 \hat{n} \times \vec{S}_1 \cdot \vec{v}_2 - 8 \vec{v}_1 \cdot \vec{v}_2 \hat{n} \cdot \vec{v}_2 \vec{S}_1 \times \vec{v}_1 \cdot \vec{v}_2 - 32 \vec{v}_1 \cdot \vec{v}_2 \hat{n} \cdot \vec{v}_1 \hat{n} \cdot \vec{v}_2 \hat{n} \times \vec{S}_1 \cdot \vec{v}_2 - \right. \\ & \left. 8 \vec{v}_2 \cdot \vec{v}_2 \vec{v}_1 \cdot \vec{v}_2 \hat{n} \times \vec{S}_1 \cdot \vec{v}_1 - 8 \vec{v}_2 \cdot \vec{v}_2 \hat{n} \cdot \vec{v}_1 \vec{S}_1 \times \vec{v}_1 \cdot \vec{v}_2 + 32 \vec{v}_2 \cdot \vec{v}_2 \hat{n} \cdot \vec{v}_1 \hat{n} \cdot \vec{v}_2 \hat{n} \times \vec{S}_1 \cdot \vec{v}_1 \right) \} \end{aligned}$$

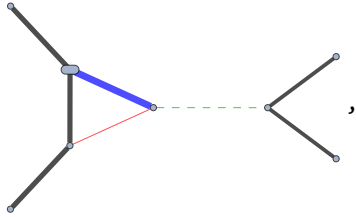

Printed by Wolfram Mathematica Student Edition



{DiagSet[2, 2, 39],

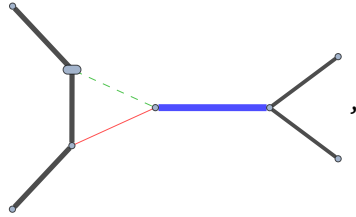

$$\frac{1}{r^2} G^2 m_1 m_2 \left( \hat{n} \cdot \vec{a}_1 \hat{n} \cdot \vec{v}_2 \vec{S}_1 \times \vec{v}_1 \cdot \vec{v}_2 + \hat{n} \cdot \vec{v}_1 \hat{n} \cdot \vec{v}_2 \vec{S}_1 \times \vec{a}_1 \cdot \vec{v}_2 + 3 \vec{a}_1 \cdot \vec{v}_2 \hat{n} \cdot \vec{v}_2 \hat{n} \times \vec{S}_1 \cdot \vec{v}_1 - 18 \vec{v}_1 \cdot \vec{a}_1 \hat{n} \cdot \vec{v}_2 \hat{n} \times \vec{S}_1 \cdot \vec{v}_2 + \right. \\ \left. 3 \vec{v}_1 \cdot \vec{v}_2 \hat{n} \cdot \vec{v}_2 \hat{n} \times \vec{S}_1 \cdot \vec{a}_1 - 4 \vec{a}_1 \cdot \vec{v}_2 \vec{S}_1 \times \vec{v}_1 \cdot \vec{v}_2 - 4 \vec{v}_1 \cdot \vec{v}_2 \vec{S}_1 \times \vec{a}_1 \cdot \vec{v}_2 + \hat{n} \cdot \vec{v}_1 \hat{n} \cdot \vec{v}_2 \vec{S}_1 \times \vec{v}_1 \cdot \vec{v}_2 + \right. \\ \left. 3 \vec{v}_1 \cdot \vec{v}_1 \hat{n} \cdot \vec{v}_2 \hat{n} \times \vec{S}_1 \cdot \vec{v}_2 + 3 \vec{v}_1 \cdot \vec{v}_2 \hat{n} \cdot \vec{v}_2 \hat{n} \times \vec{S}_1 \cdot \vec{v}_1 + \vec{v}_2 \cdot \vec{v}_2 \hat{n} \cdot \vec{v}_2 \hat{n} \times \vec{S}_1 \cdot \vec{v}_2 - 4 \vec{v}_1 \cdot \vec{v}_2 \vec{S}_1 \times \vec{v}_1 \cdot \vec{v}_2 \right) + \\ \frac{G^2 m_1 m_2 \left( -16 \hat{n} \cdot \vec{v}_2 \vec{S}_1 \times \vec{a}_1 \cdot \vec{v}_2 - 8 \hat{n} \cdot \vec{v}_2 \vec{S}_1 \times \vec{a}_1 \cdot \vec{v}_2 - 8 \hat{n} \cdot \vec{v}_2 \vec{S}_1 \times \vec{v}_1 \cdot \vec{v}_2 \right)}{r} + \frac{1}{r^3} \\ G^2 m_1 m_2 \left( 2 \vec{v}_1 \cdot \vec{v}_1 \hat{n} \cdot \vec{v}_2 \vec{S}_1 \times \vec{v}_1 \cdot \vec{v}_2 + 4 \vec{v}_1 \cdot \vec{v}_2 \hat{n} \cdot \vec{v}_1 \vec{S}_1 \times \vec{v}_1 \cdot \vec{v}_2 + \vec{v}_2 \cdot \vec{v}_2 \hat{n} \cdot \vec{v}_2 \vec{S}_1 \times \vec{v}_1 \cdot \vec{v}_2 \right) \Big\}$$

{DiagSet[2, 2, 40],

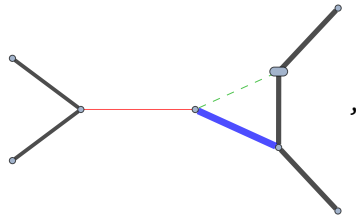

$$\frac{1}{r^2} G^2 m_1 m_2 \left( 20 (\hat{n} \cdot \vec{v}_1)^2 \vec{S}_1 \times \vec{v}_1 \cdot \vec{a}_1 - 16 \hat{n} \cdot \vec{v}_2 \hat{n} \cdot \vec{v}_1 \vec{S}_1 \times \vec{v}_1 \cdot \vec{a}_1 - 12 \vec{v}_1 \cdot \vec{a}_1 \hat{n} \cdot \vec{v}_1 \hat{n} \times \vec{S}_1 \cdot \vec{v}_1 - 12 \vec{v}_1 \cdot \vec{v}_1 \hat{n} \cdot \vec{v}_1 \hat{n} \times \vec{S}_1 \cdot \vec{a}_1 - \right. \\ \left. 18 \vec{v}_2 \cdot \vec{a}_2 \hat{n} \cdot \vec{v}_1 \hat{n} \times \vec{S}_1 \cdot \vec{v}_1 - 16 \vec{v}_1 \cdot \vec{v}_1 \vec{S}_1 \times \vec{v}_1 \cdot \vec{a}_1 + 8 \vec{v}_1 \cdot \vec{v}_2 \vec{S}_1 \times \vec{v}_1 \cdot \vec{a}_1 - 16 \vec{v}_1 \cdot \vec{v}_1 \hat{n} \cdot \vec{v}_1 \hat{n} \times \vec{S}_1 \cdot \vec{v}_1 - \right. \\ \left. 12 \vec{v}_2 \cdot \vec{v}_2 \hat{n} \cdot \vec{v}_1 \hat{n} \times \vec{S}_1 \cdot \vec{v}_1 \right) + \frac{G^2 m_1 m_2 \left( -32 \hat{n} \cdot \vec{v}_1 \vec{S}_1 \times \vec{v}_1 \cdot \vec{a}_1 - 16 \hat{n} \cdot \vec{v}_1 \vec{S}_1 \times \vec{v}_1 \cdot \vec{a}_1 \right)}{r} + \frac{1}{r^3} \\ G^2 m_1 m_2 \left( 48 \vec{v}_1 \cdot \vec{v}_1 (\hat{n} \cdot \vec{v}_1)^2 \hat{n} \times \vec{S}_1 \cdot \vec{v}_1 + 36 \vec{v}_2 \cdot \vec{v}_2 (\hat{n} \cdot \vec{v}_1)^2 \hat{n} \times \vec{S}_1 \cdot \vec{v}_1 + 12 \vec{v}_1 \cdot \vec{v}_1 \hat{n} \cdot \vec{v}_1 \vec{S}_1 \times \vec{v}_1 \cdot \vec{v}_2 - \right. \\ \left. 48 \vec{v}_1 \cdot \vec{v}_1 \hat{n} \cdot \vec{v}_2 \hat{n} \cdot \vec{v}_1 \hat{n} \times \vec{S}_1 \cdot \vec{v}_1 + 9 \vec{v}_2 \cdot \vec{v}_2 \hat{n} \cdot \vec{v}_1 \vec{S}_1 \times \vec{v}_1 \cdot \vec{v}_2 - 36 \vec{v}_2 \cdot \vec{v}_2 \hat{n} \cdot \vec{v}_2 \hat{n} \cdot \vec{v}_1 \hat{n} \times \vec{S}_1 \cdot \vec{v}_1 - \right. \\ \left. 12 (\vec{v}_1 \cdot \vec{v}_1)^2 \hat{n} \times \vec{S}_1 \cdot \vec{v}_1 + 12 \vec{v}_1 \cdot \vec{v}_1 \vec{v}_1 \cdot \vec{v}_2 \hat{n} \times \vec{S}_1 \cdot \vec{v}_1 - 9 \vec{v}_1 \cdot \vec{v}_1 \vec{v}_2 \cdot \vec{v}_2 \hat{n} \times \vec{S}_1 \cdot \vec{v}_1 + 9 \vec{v}_1 \cdot \vec{v}_2 \vec{v}_2 \cdot \vec{v}_2 \hat{n} \times \vec{S}_1 \cdot \vec{v}_1 \right) \Big\}$$

{DiagSet[2, 2, 41],

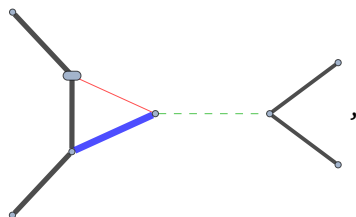

$$\frac{1}{r^2} G^2 m_1 m_2 \left( 24 \vec{v}_1 \cdot \vec{a}_2 \hat{n} \cdot \vec{v}_1 \hat{n} \times \vec{S}_1 \cdot \vec{v}_1 + 32 \vec{v}_1 \cdot \vec{v}_2 \hat{n} \cdot \vec{v}_1 \hat{n} \times \vec{S}_1 \cdot \vec{a}_1 + 16 \vec{v}_1 \cdot \vec{v}_2 \vec{S}_1 \times \vec{v}_1 \cdot \vec{a}_1 + 32 \vec{v}_1 \cdot \vec{v}_2 \hat{n} \cdot \vec{v}_1 \hat{n} \times \vec{S}_1 \cdot \vec{v}_1 \right) + \\ \frac{1}{r^3} G^2 m_1 m_2 \left( -96 \vec{v}_1 \cdot \vec{v}_2 (\hat{n} \cdot \vec{v}_1)^2 \hat{n} \times \vec{S}_1 \cdot \vec{v}_1 - 24 \vec{v}_1 \cdot \vec{v}_2 \hat{n} \cdot \vec{v}_1 \vec{S}_1 \times \vec{v}_1 \cdot \vec{v}_2 + \right. \\ \left. 96 \vec{v}_1 \cdot \vec{v}_2 \hat{n} \cdot \vec{v}_2 \hat{n} \cdot \vec{v}_1 \hat{n} \times \vec{S}_1 \cdot \vec{v}_1 - 24 (\vec{v}_1 \cdot \vec{v}_2)^2 \hat{n} \times \vec{S}_1 \cdot \vec{v}_1 + 24 \vec{v}_1 \cdot \vec{v}_1 \vec{v}_1 \cdot \vec{v}_2 \hat{n} \times \vec{S}_1 \cdot \vec{v}_1 \right) \Big\}$$

{DiagSet[2, 2, 42],

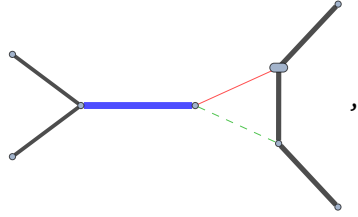

,

$$\frac{1}{r^2} G^2 m_1 m_2 \left( 24 \vec{a}_1 \cdot \vec{v}_2 \hat{n} \cdot \vec{v}_2 \hat{n} \cdot \vec{S}_1 \cdot \vec{v}_1 - 8 \vec{v}_1 \cdot \vec{v}_2 \hat{n} \cdot \vec{v}_2 \hat{n} \cdot \vec{S}_1 \cdot \vec{a}_1 - 8 \vec{a}_1 \cdot \vec{v}_2 \vec{S}_1 \times \vec{v}_1 \cdot \vec{v}_2 + \right. \\ \left. 8 \vec{v}_1 \cdot \vec{v}_2 \vec{S}_1 \times \vec{a}_1 \cdot \vec{v}_2 - 8 \vec{v}_1 \cdot \vec{v}_2 \hat{n} \cdot \vec{v}_2 \hat{n} \cdot \vec{S}_1 \cdot \vec{v}_1 + 8 \vec{v}_1 \cdot \vec{v}_2 \vec{S}_1 \times \vec{v}_1 \cdot \vec{v}_2 \right) - \frac{8 G^2 m_1 m_2 \vec{v}_1 \cdot \vec{v}_2 \hat{n} \cdot \vec{v}_1 \vec{S}_1 \times \vec{v}_1 \cdot \vec{v}_2}{r^3} \Bigg\}$$

{DiagSet[2, 2, 43],

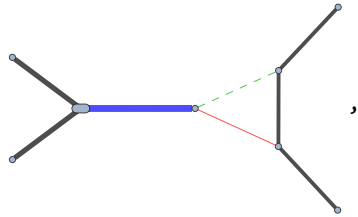

,

$$\frac{1}{r^2} G^2 m_2^2 \left( -4 (\hat{n} \cdot \vec{v}_1)^2 \vec{a}_2 \times \vec{S}_1 \cdot \vec{v}_1 - 12 \vec{a}_2 \cdot \vec{v}_1 \hat{n} \cdot \vec{v}_1 \hat{n} \cdot \vec{S}_1 \cdot \vec{v}_1 + 16 \vec{a}_2 \cdot \vec{v}_2 \hat{n} \cdot \vec{v}_1 \hat{n} \cdot \vec{S}_1 \cdot \vec{v}_2 + 16 \vec{v}_2 \cdot \vec{v}_2 \hat{n} \cdot \vec{v}_1 \hat{n} \cdot \vec{a}_2 \cdot \vec{S}_1 + \right. \\ \left. 8 \vec{a}_2 \cdot \vec{v}_2 \vec{S}_1 \times \vec{v}_1 \cdot \vec{v}_2 + 2 \vec{v}_1 \cdot \vec{v}_1 \vec{a}_2 \times \vec{S}_1 \cdot \vec{v}_1 - 8 \vec{v}_2 \cdot \vec{v}_2 \vec{a}_2 \times \vec{S}_1 \cdot \vec{v}_1 \right) + \frac{1}{r} G^2 m_2^2 \left( 4 \hat{n} \cdot \vec{a}_1 \vec{a}_2 \times \vec{S}_1 \cdot \vec{v}_1 + \right. \\ \left. 8 \hat{n} \cdot \vec{v}_1 \vec{a}_1 \times \vec{a}_2 \cdot \vec{S}_1 + 6 \hat{n} \cdot \vec{v}_1 \vec{a}_2 \times \vec{S}_1 \cdot \vec{v}_1 + 4 \vec{a}_1 \cdot \vec{a}_2 \hat{n} \cdot \vec{S}_1 \cdot \vec{v}_1 + 6 \vec{a}_2 \cdot \vec{v}_1 \hat{n} \times \vec{S}_1 \cdot \vec{v}_1 - 8 \vec{a}_2 \cdot \vec{v}_1 \hat{n} \times \vec{a}_1 \cdot \vec{S}_1 \right) \Bigg\}$$

{DiagSet[2, 2, 44],

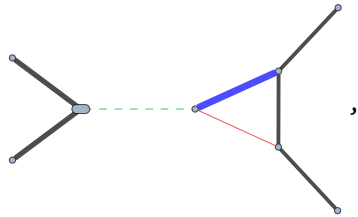

,

$$G^2 \left( -8 \frac{1}{r} \vec{a}_1 \times \vec{S}_1 \cdot \vec{v}_2 \hat{n} \cdot \vec{v}_2 + 8 \vec{S}_1 \times \vec{v}_1 \cdot \vec{v}_2 \hat{n} \cdot \vec{v}_2 - 16 \vec{a}_1 \times \vec{S}_1 \cdot \vec{v}_2 \hat{n} \cdot \vec{v}_2 \right) m_2^2 + \frac{1}{r^2} \\ G^2 \left( 16 \vec{S}_1 \times \vec{v}_1 \cdot \vec{v}_2 (\hat{n} \cdot \vec{v}_2)^2 - 16 \vec{a}_1 \times \vec{S}_1 \cdot \vec{v}_2 (\hat{n} \cdot \vec{v}_2)^2 - 4 \vec{S}_1 \times \vec{v}_1 \cdot \vec{v}_2 \hat{n} \cdot \vec{a}_1 \hat{n} \cdot \vec{v}_2 - 20 \vec{S}_1 \times \vec{v}_1 \cdot \vec{v}_2 \hat{n} \cdot \vec{v}_1 \hat{n} \cdot \vec{v}_2 + \right. \\ \left. 20 \vec{a}_1 \times \vec{S}_1 \cdot \vec{v}_2 \hat{n} \cdot \vec{v}_1 \hat{n} \cdot \vec{v}_2 - 12 \hat{n} \cdot \vec{S}_1 \cdot \vec{v}_1 \vec{a}_1 \cdot \vec{v}_2 \hat{n} \cdot \vec{v}_2 - 48 \hat{n} \times \vec{S}_1 \cdot \vec{v}_2 \vec{a}_2 \cdot \vec{v}_2 \hat{n} \cdot \vec{v}_2 - \right. \\ \left. 12 \hat{n} \times \vec{S}_1 \cdot \vec{v}_1 \vec{v}_1 \cdot \vec{v}_2 \hat{n} \cdot \vec{v}_2 + 12 \hat{n} \times \vec{a}_1 \cdot \vec{S}_1 \vec{v}_1 \cdot \vec{v}_2 \hat{n} \cdot \vec{v}_2 - 16 \hat{n} \times \vec{S}_1 \cdot \vec{v}_2 \vec{v}_2 \cdot \vec{v}_2 \hat{n} \cdot \vec{v}_2 + 8 \vec{S}_1 \times \vec{v}_1 \cdot \vec{v}_2 \vec{a}_1 \cdot \vec{v}_2 + \right. \\ \left. 16 \vec{S}_1 \times \vec{v}_1 \cdot \vec{v}_2 \vec{v}_1 \cdot \vec{v}_2 - 16 \vec{a}_1 \times \vec{S}_1 \cdot \vec{v}_2 \vec{v}_1 \cdot \vec{v}_2 - 8 \vec{S}_1 \times \vec{v}_1 \cdot \vec{v}_2 \vec{v}_2 \cdot \vec{v}_2 + 8 \vec{a}_1 \times \vec{S}_1 \cdot \vec{v}_2 \vec{v}_2 \cdot \vec{v}_2 \right) m_2^2 + \\ \frac{1}{r^3} G^2 \left( 16 \vec{S}_1 \times \vec{v}_1 \cdot \vec{v}_2 \hat{n} \cdot \vec{v}_2 (\hat{n} \cdot \vec{v}_1)^2 - 16 \vec{S}_1 \times \vec{v}_1 \cdot \vec{v}_2 (\hat{n} \cdot \vec{v}_2)^2 \hat{n} \cdot \vec{v}_1 - 20 \vec{S}_1 \times \vec{v}_1 \cdot \vec{v}_2 \vec{v}_1 \cdot \vec{v}_2 \hat{n} \cdot \vec{v}_1 + \right. \\ \left. 48 \hat{n} \times \vec{S}_1 \cdot \vec{v}_1 \hat{n} \cdot \vec{v}_2 \vec{v}_1 \cdot \vec{v}_2 \hat{n} \cdot \vec{v}_1 + 4 \vec{S}_1 \times \vec{v}_1 \cdot \vec{v}_2 \vec{v}_2 \cdot \vec{v}_2 \hat{n} \cdot \vec{v}_1 + 64 \hat{n} \times \vec{S}_1 \cdot \vec{v}_2 \hat{n} \cdot \vec{v}_2 \vec{v}_2 \cdot \vec{v}_2 \hat{n} \cdot \vec{v}_1 - \right. \\ \left. 12 \hat{n} \times \vec{S}_1 \cdot \vec{v}_1 (\vec{v}_1 \cdot \vec{v}_2)^2 + 16 \hat{n} \times \vec{S}_1 \cdot \vec{v}_2 (\vec{v}_2 \cdot \vec{v}_2)^2 - 4 \vec{S}_1 \times \vec{v}_1 \cdot \vec{v}_2 \hat{n} \cdot \vec{v}_2 \vec{v}_1 \cdot \vec{v}_1 - \right. \\ \left. 48 \hat{n} \times \vec{S}_1 \cdot \vec{v}_1 (\hat{n} \cdot \vec{v}_2)^2 \vec{v}_1 \cdot \vec{v}_2 + 32 \vec{S}_1 \times \vec{v}_1 \cdot \vec{v}_2 \hat{n} \cdot \vec{v}_2 \vec{v}_1 \cdot \vec{v}_2 - 64 \hat{n} \times \vec{S}_1 \cdot \vec{v}_2 (\hat{n} \cdot \vec{v}_2)^2 \vec{v}_2 \cdot \vec{v}_2 + \right. \\ \left. 16 \vec{S}_1 \times \vec{v}_1 \cdot \vec{v}_2 \hat{n} \cdot \vec{v}_2 \vec{v}_2 \cdot \vec{v}_2 + 12 \hat{n} \times \vec{S}_1 \cdot \vec{v}_1 \vec{v}_1 \cdot \vec{v}_2 \vec{v}_2 \cdot \vec{v}_2 - 16 \hat{n} \times \vec{S}_1 \cdot \vec{v}_2 \vec{v}_1 \cdot \vec{v}_2 \vec{v}_2 \cdot \vec{v}_2 \right) m_2^2 \Bigg\}$$

{DiagSet[2, 2, 45],

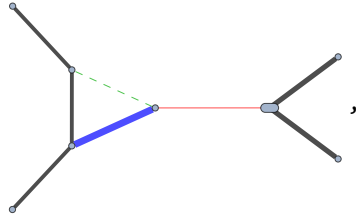

$$\frac{1}{r^2} G^2 m_2^2 \left( 64 \vec{a}_2 \cdot \vec{v}_2 \hat{n} \cdot \vec{v}_2 \hat{n} \cdot \vec{S}_1 \cdot \vec{v}_1 - 32 \vec{v}_2 \cdot \vec{v}_2 \hat{n} \cdot \vec{v}_2 \hat{n} \times \vec{a}_1 \cdot \vec{S}_1 - 32 \vec{a}_2 \cdot \vec{v}_2 \vec{S}_1 \times \vec{v}_1 \cdot \vec{v}_2 + \right. \\ \left. 16 \vec{v}_2 \cdot \vec{v}_2 \vec{a}_1 \times \vec{S}_1 \cdot \vec{v}_2 + 32 \vec{v}_2 \cdot \vec{v}_2 \hat{n} \cdot \vec{v}_2 \hat{n} \times \vec{S}_1 \cdot \vec{v}_1 - 16 \vec{v}_2 \cdot \vec{v}_2 \vec{S}_1 \times \vec{v}_1 \cdot \vec{v}_2 \right) + \frac{1}{r^3} \\ G^2 m_2^2 \left( 128 \vec{v}_2 \cdot \vec{v}_2 (\hat{n} \cdot \vec{v}_2)^2 \hat{n} \times \vec{S}_1 \cdot \vec{v}_1 - 64 \vec{v}_2 \cdot \vec{v}_2 \hat{n} \cdot \vec{v}_2 \vec{S}_1 \times \vec{v}_1 \cdot \vec{v}_2 - 128 \vec{v}_2 \cdot \vec{v}_2 \hat{n} \cdot \vec{v}_1 \hat{n} \cdot \vec{v}_2 \hat{n} \times \vec{S}_1 \cdot \vec{v}_1 - \right. \\ \left. 32 (\vec{v}_2 \cdot \vec{v}_2)^2 \hat{n} \times \vec{S}_1 \cdot \vec{v}_1 + 32 \vec{v}_2 \cdot \vec{v}_2 \hat{n} \cdot \vec{v}_1 \vec{S}_1 \times \vec{v}_1 \cdot \vec{v}_2 + 32 \vec{v}_1 \cdot \vec{v}_2 \vec{v}_2 \cdot \vec{v}_2 \hat{n} \times \vec{S}_1 \cdot \vec{v}_1 \right) \Big\}$$

{DiagSet[2, 2, 46],

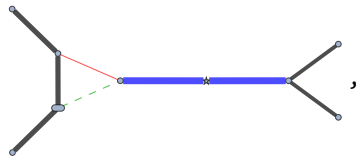

$$\frac{1}{r^2} G^2 m_1 m_2 \left( 2 (\hat{n} \cdot \vec{v}_2)^2 \vec{S}_1 \times \vec{a}_1 \cdot \vec{v}_2 - 2 \hat{n} \cdot \vec{v}_1 \hat{n} \cdot \vec{v}_2 \vec{S}_1 \times \vec{v}_1 \cdot \vec{a}_2 - 2 \hat{n} \cdot \vec{a}_2 \hat{n} \cdot \vec{v}_1 \vec{S}_1 \times \vec{v}_1 \cdot \vec{v}_2 + \vec{v}_1 \cdot \vec{a}_2 \vec{S}_1 \times \vec{v}_1 \cdot \vec{v}_2 + \right. \\ \left. \vec{v}_1 \cdot \vec{v}_2 \vec{S}_1 \times \vec{v}_1 \cdot \vec{a}_2 - \vec{v}_2 \cdot \vec{v}_2 \vec{S}_1 \times \vec{a}_1 \cdot \vec{v}_2 + \frac{4}{3} (\hat{n} \cdot \vec{v}_2)^2 \vec{S}_1 \times \vec{v}_1 \cdot \vec{v}_2 - \frac{8}{3} \hat{n} \cdot \vec{v}_1 (\hat{n} \cdot \vec{v}_2)^2 \hat{n} \times \vec{S}_1 \cdot \vec{v}_2 + \right. \\ \left. \frac{4}{3} \vec{v}_1 \cdot \vec{v}_2 \hat{n} \cdot \vec{v}_2 \hat{n} \times \vec{S}_1 \cdot \vec{v}_2 + \frac{2}{3} \vec{v}_2 \cdot \vec{v}_2 \hat{n} \cdot \vec{v}_1 \hat{n} \times \vec{S}_1 \cdot \vec{v}_2 - \frac{2}{3} \vec{v}_2 \cdot \vec{v}_2 \vec{S}_1 \times \vec{v}_1 \cdot \vec{v}_2 \right) + \frac{1}{r} \\ G^2 m_1 m_2 \left( \frac{2}{3} \hat{n} \cdot \vec{v}_2 \vec{S}_1 \times \vec{v}_1 \cdot \vec{a}_2 + \hat{n} \cdot \vec{v}_2 \vec{S}_1 \times \vec{a}_1 \cdot \vec{a}_2 - \frac{2}{3} \hat{n} \cdot \vec{v}_1 \hat{n} \cdot \vec{v}_2 \hat{n} \times \vec{S}_1 \cdot \vec{a}_2 + \frac{2}{3} \hat{n} \cdot \vec{a}_2 \vec{S}_1 \times \vec{v}_1 \cdot \vec{v}_2 + \hat{n} \cdot \vec{a}_2 \vec{S}_1 \times \vec{a}_1 \cdot \vec{v}_2 - \right. \\ \left. \frac{2}{3} \hat{n} \cdot \vec{a}_2 \hat{n} \cdot \vec{v}_1 \hat{n} \times \vec{S}_1 \cdot \vec{v}_2 + \frac{1}{3} \vec{v}_1 \cdot \vec{a}_2 \hat{n} \times \vec{S}_1 \cdot \vec{v}_2 + \frac{1}{3} \vec{v}_1 \cdot \vec{v}_2 \hat{n} \times \vec{S}_1 \cdot \vec{a}_2 + \frac{2}{3} (\hat{n} \cdot \vec{v}_2)^2 \hat{n} \times \vec{S}_1 \cdot \vec{v}_2 - \frac{1}{3} \vec{v}_2 \cdot \vec{v}_2 \hat{n} \times \vec{S}_1 \cdot \vec{v}_2 \right) + \\ G^2 m_1 m_2 \left( \frac{1}{3} \hat{n} \cdot \vec{a}_2 \hat{n} \times \vec{S}_1 \cdot \vec{v}_2 + \frac{1}{3} \hat{n} \cdot \vec{v}_2 \hat{n} \times \vec{S}_1 \cdot \vec{a}_2 \right) + \frac{1}{r^3} \\ G^2 m_1 m_2 \left( -8 \hat{n} \cdot \vec{v}_1 (\hat{n} \cdot \vec{v}_2)^2 \vec{S}_1 \times \vec{v}_1 \cdot \vec{v}_2 + 4 \vec{v}_1 \cdot \vec{v}_2 \hat{n} \cdot \vec{v}_2 \vec{S}_1 \times \vec{v}_1 \cdot \vec{v}_2 + 2 \vec{v}_2 \cdot \vec{v}_2 \hat{n} \cdot \vec{v}_1 \vec{S}_1 \times \vec{v}_1 \cdot \vec{v}_2 \right) \Big\}$$

{DiagSet[2, 2, 47],

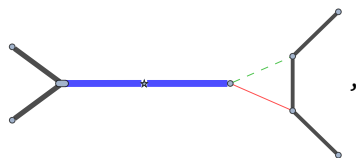

$$G^2 m_2^2 \left( \frac{-\frac{2}{3} \frac{1}{\vec{a}_2} \times \vec{S}_1 \cdot \vec{v}_1 - \frac{2}{3} \vec{a}_1 \times \frac{1}{\vec{a}_2} \cdot \vec{S}_1}{\epsilon_d} + \frac{4}{3} \hat{n} \cdot \vec{v}_1 \hat{n} \times \frac{1}{\vec{a}_2} \cdot \vec{S}_1 + \frac{4}{3} \hat{n} \cdot \vec{a}_1 \hat{n} \times \frac{1}{\vec{a}_2} \cdot \vec{S}_1 + \right. \\ \left. \frac{4}{3} \log\left(\frac{r}{R_\theta}\right) \frac{1}{\vec{a}_2} \times \vec{S}_1 \cdot \vec{v}_1 + \frac{4}{3} \log\left(\frac{r}{R_\theta}\right) \vec{a}_1 \times \frac{1}{\vec{a}_2} \cdot \vec{S}_1 - \frac{8}{9} \frac{1}{\vec{a}_2} \times \vec{S}_1 \cdot \vec{v}_1 - \frac{8}{9} \vec{a}_1 \times \frac{1}{\vec{a}_2} \cdot \vec{S}_1 \right) + \\ \frac{1}{r^2} G^2 m_2^2 \left( \frac{8}{3} (\hat{n} \cdot \vec{v}_1)^2 \vec{a}_2 \times \vec{S}_1 \cdot \vec{v}_2 - \frac{32}{3} \hat{n} \cdot \vec{v}_2 (\hat{n} \cdot \vec{v}_1)^2 \hat{n} \times \vec{a}_2 \cdot \vec{S}_1 + \frac{16}{3} \hat{n} \cdot \vec{v}_2 \hat{n} \cdot \vec{v}_1 \vec{a}_2 \times \vec{S}_1 \cdot \vec{v}_1 + \right. \\ \left. \frac{16}{3} \vec{v}_1 \cdot \vec{v}_2 \hat{n} \cdot \vec{v}_1 \hat{n} \times \vec{a}_2 \cdot \vec{S}_1 + \frac{8}{3} \vec{v}_1 \cdot \vec{v}_1 \hat{n} \cdot \vec{v}_2 \hat{n} \times \vec{a}_2 \cdot \vec{S}_1 - \frac{4}{3} \vec{v}_1 \cdot \vec{v}_1 \vec{a}_2 \times \vec{S}_1 \cdot \vec{v}_2 - \frac{8}{3} \vec{v}_1 \cdot \vec{v}_2 \vec{a}_2 \times \vec{S}_1 \cdot \vec{v}_1 \right) +$$

`diagSet[2, 2, 48]`, 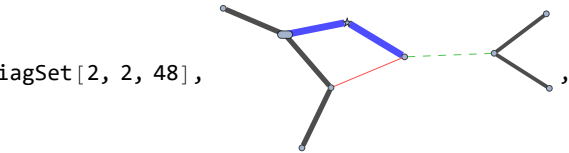

Printed by Wolfram Mathematica Student Edition

$$\begin{aligned}
 & \frac{20}{3} \vec{S}_1 \times \vec{v}_1 \cdot \vec{v}_2 \vec{v}_1 \cdot \vec{v}_2 - \frac{1}{3} \vec{S}_1 \times \vec{a}_1 \cdot \vec{v}_2 \vec{v}_1 \cdot \vec{v}_2 - 2 \vec{S}_1 \times \vec{v}_1 \cdot \vec{a}_1 \vec{v}_1 \cdot \vec{v}_2 + \frac{14}{3} \vec{S}_1 \times \vec{v}_1 \cdot \vec{a}_2 \vec{v}_1 \cdot \vec{v}_2 + \\
 & 3 \hat{n} \times \vec{S}_1 \cdot \vec{v}_1 \hat{n} \cdot \vec{a}_1 \vec{v}_1 \cdot \vec{v}_2 + \frac{7}{3} \hat{n} \times \vec{S}_1 \cdot \vec{v}_2 \hat{n} \cdot \vec{a}_1 \vec{v}_1 \cdot \vec{v}_2 - 4 \hat{n} \times \vec{S}_1 \cdot \vec{v}_1 \hat{n} \cdot \vec{a}_2 \vec{v}_1 \cdot \vec{v}_2 + 8 \hat{n} \times \vec{S}_1 \cdot \vec{v}_1 \hat{n} \cdot \vec{v}_2 \vec{v}_1 \cdot \vec{v}_2 - \\
 & \frac{8}{3} \hat{n} \times \vec{S}_1 \cdot \vec{v}_2 \hat{n} \cdot \vec{v}_2 \vec{v}_1 \cdot \vec{v}_2 + \frac{4}{3} \vec{S}_1 \times \vec{v}_1 \cdot \vec{v}_2 \vec{v}_2 \cdot \vec{v}_2 + \frac{4}{3} \vec{S}_1 \times \vec{a}_1 \cdot \vec{v}_2 \vec{v}_2 \cdot \vec{v}_2 - \frac{4}{3} \hat{n} \times \vec{S}_1 \cdot \vec{v}_2 \hat{n} \cdot \vec{a}_1 \vec{v}_2 \cdot \vec{v}_2 \Big) m_1 m_2 G^2 + \frac{1}{r^3} \\
 & \left( -4 \hat{n} \times \vec{S}_1 \cdot \vec{v}_2 (\hat{n} \cdot \vec{v}_1)^4 - \frac{26}{3} \vec{S}_1 \times \vec{v}_1 \cdot \vec{v}_2 (\hat{n} \cdot \vec{v}_1)^3 + 12 \hat{n} \times \vec{S}_1 \cdot \vec{v}_2 \hat{n} \cdot \vec{v}_2 (\hat{n} \cdot \vec{v}_1)^3 - 8 \hat{n} \times \vec{S}_1 \cdot \vec{v}_2 (\hat{n} \cdot \vec{v}_2)^2 (\hat{n} \cdot \vec{v}_1)^2 + \right. \\
 & 20 \vec{S}_1 \times \vec{v}_1 \cdot \vec{v}_2 \hat{n} \cdot \vec{v}_2 (\hat{n} \cdot \vec{v}_1)^2 + 2 \hat{n} \times \vec{S}_1 \cdot \vec{v}_2 \vec{v}_1 \cdot \vec{v}_1 (\hat{n} \cdot \vec{v}_1)^2 - 6 \hat{n} \times \vec{S}_1 \cdot \vec{v}_1 \vec{v}_1 \cdot \vec{v}_2 (\hat{n} \cdot \vec{v}_1)^2 - \\
 & 6 \hat{n} \times \vec{S}_1 \cdot \vec{v}_2 \vec{v}_1 \cdot \vec{v}_2 (\hat{n} \cdot \vec{v}_1)^2 + \frac{4}{3} \hat{n} \times \vec{S}_1 \cdot \vec{v}_2 \vec{v}_2 \cdot \vec{v}_2 (\hat{n} \cdot \vec{v}_1)^2 - \frac{32}{3} \vec{S}_1 \times \vec{v}_1 \cdot \vec{v}_2 (\hat{n} \cdot \vec{v}_2)^2 \hat{n} \cdot \vec{v}_1 + \\
 & 4 \vec{S}_1 \times \vec{v}_1 \cdot \vec{v}_2 \vec{v}_1 \cdot \vec{v}_1 \hat{n} \cdot \vec{v}_1 - 14 \vec{S}_1 \times \vec{v}_1 \cdot \vec{v}_2 \vec{v}_1 \cdot \vec{v}_2 \hat{n} \cdot \vec{v}_1 + 16 \hat{n} \times \vec{S}_1 \cdot \vec{v}_1 \hat{n} \cdot \vec{v}_2 \vec{v}_1 \cdot \vec{v}_2 \hat{n} \cdot \vec{v}_1 + \\
 & \frac{16}{3} \hat{n} \times \vec{S}_1 \cdot \vec{v}_2 \hat{n} \cdot \vec{v}_2 \vec{v}_1 \cdot \vec{v}_2 \hat{n} \cdot \vec{v}_1 + \frac{8}{3} \vec{S}_1 \times \vec{v}_1 \cdot \vec{v}_2 \vec{v}_2 \cdot \vec{v}_2 \hat{n} \cdot \vec{v}_1 - 4 \hat{n} \times \vec{S}_1 \cdot \vec{v}_1 (\vec{v}_1 \cdot \vec{v}_2)^2 - \frac{2}{3} \hat{n} \times \vec{S}_1 \cdot \vec{v}_2 (\vec{v}_1 \cdot \vec{v}_2)^2 - \\
 & \frac{8}{3} \hat{n} \times \vec{S}_1 \cdot \vec{v}_2 (\hat{n} \cdot \vec{v}_2)^2 \vec{v}_1 \cdot \vec{v}_1 - 2 \vec{S}_1 \times \vec{v}_1 \cdot \vec{v}_2 \hat{n} \cdot \vec{v}_2 \vec{v}_1 \cdot \vec{v}_1 - 16 \hat{n} \times \vec{S}_1 \cdot \vec{v}_1 (\hat{n} \cdot \vec{v}_2)^2 \vec{v}_1 \cdot \vec{v}_2 + \\
 & \left. \frac{40}{3} \vec{S}_1 \times \vec{v}_1 \cdot \vec{v}_2 \hat{n} \cdot \vec{v}_2 \vec{v}_1 \cdot \vec{v}_2 + \frac{2}{3} \hat{n} \times \vec{S}_1 \cdot \vec{v}_2 \vec{v}_1 \cdot \vec{v}_1 \vec{v}_2 \cdot \vec{v}_2 + 4 \hat{n} \times \vec{S}_1 \cdot \vec{v}_1 \vec{v}_1 \cdot \vec{v}_2 \vec{v}_2 \cdot \vec{v}_2 \right) m_1 m_2 G^2 + \\
 & m_1 m_2 \left( \frac{4}{3} \log \left( \frac{r}{R_\theta} \right) \vec{S}_1 \times \vec{v}_1 \cdot \vec{a}_2 - \frac{8}{9} \vec{S}_1 \times \vec{v}_1 \cdot \vec{a}_2 - \frac{8}{9} \vec{S}_1 \times \vec{a}_1 \cdot \vec{a}_2 + \frac{2}{3} \hat{n} \times \vec{S}_1 \cdot \vec{a}_2 \hat{n} \cdot \vec{a}_1 + \right. \\
 & \left. \frac{2}{3} \hat{n} \times \vec{S}_1 \cdot \vec{a}_2 \hat{n} \cdot \vec{v}_1 + \frac{4}{3} \vec{S}_1 \times \vec{a}_1 \cdot \vec{a}_2 \log \left( \frac{r}{R_\theta} \right) + \frac{-\frac{2}{3} \vec{S}_1 \times \vec{v}_1 \cdot \vec{a}_2 - \frac{2}{3} \vec{S}_1 \times \vec{a}_1 \cdot \vec{a}_2}{\epsilon_d} \right) G^2 \Big\}
 \end{aligned}$$

{DiagSet[2, 2, 49],

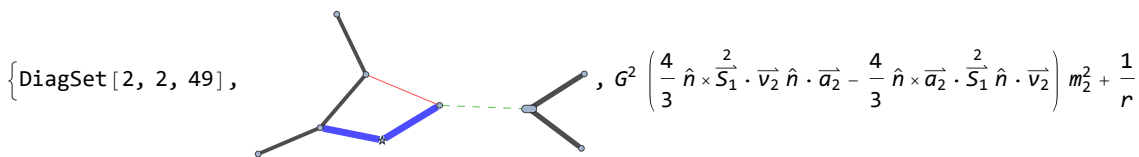

,  $G^2 \left( \frac{4}{3} \hat{n} \times \vec{S}_1 \cdot \vec{v}_2 \hat{n} \cdot \vec{a}_2 - \frac{4}{3} \hat{n} \times \vec{a}_2 \cdot \vec{S}_1 \hat{n} \cdot \vec{v}_2 \right) m_2^2 + \frac{1}{r}$

$$\begin{aligned}
 & G^2 \left( \frac{8}{3} \hat{n} \times \vec{S}_1 \cdot \vec{v}_2 (\hat{n} \cdot \vec{a}_2)^2 - \frac{8}{3} \vec{S}_1 \times \vec{v}_1 \cdot \vec{v}_2 \hat{n} \cdot \vec{a}_2 + \frac{4}{3} \vec{a}_1 \times \vec{S}_1 \cdot \vec{v}_2 \hat{n} \cdot \vec{a}_2 - \frac{4}{3} \vec{a}_2 \times \vec{S}_1 \cdot \vec{v}_2 \hat{n} \cdot \vec{a}_2 - \frac{8}{3} \hat{n} \times \vec{S}_1 \cdot \vec{v}_2 \hat{n} \cdot \vec{a}_1 \hat{n} \cdot \vec{a}_2 - \right. \\
 & \frac{16}{3} \hat{n} \times \vec{S}_1 \cdot \vec{v}_2 \hat{n} \cdot \vec{v}_1 \hat{n} \cdot \vec{a}_2 + \frac{20}{3} \hat{n} \times \vec{S}_1 \cdot \vec{v}_2 \hat{n} \cdot \vec{v}_2 \hat{n} \cdot \vec{a}_2 - \frac{8}{3} \hat{n} \times \vec{a}_2 \cdot \vec{S}_1 \hat{n} \cdot \vec{v}_2 \hat{n} \cdot \vec{a}_2 - \frac{4}{3} \hat{n} \times \vec{S}_1 \cdot \vec{v}_2 (\hat{n} \cdot \vec{v}_2)^2 - \\
 & \frac{20}{3} \hat{n} \times \vec{a}_2 \cdot \vec{S}_1 (\hat{n} \cdot \vec{v}_2)^2 - \frac{4}{3} \vec{a}_1 \times \vec{a}_2 \cdot \vec{S}_1 \hat{n} \cdot \vec{v}_2 - \frac{8}{3} \vec{a}_2 \times \vec{S}_1 \cdot \vec{v}_1 \hat{n} \cdot \vec{v}_2 + \frac{10}{3} \vec{a}_2 \times \vec{S}_1 \cdot \vec{v}_2 \hat{n} \cdot \vec{v}_2 + \frac{8}{3} \hat{n} \times \vec{a}_2 \cdot \vec{S}_1 \hat{n} \cdot \vec{a}_1 \hat{n} \cdot \vec{v}_2 + \\
 & \frac{16}{3} \hat{n} \times \vec{a}_2 \cdot \vec{S}_1 \hat{n} \cdot \vec{v}_1 \hat{n} \cdot \vec{v}_2 + \frac{4}{3} \hat{n} \times \vec{S}_1 \cdot \vec{v}_2 \vec{a}_1 \cdot \vec{a}_2 - \frac{4}{3} \hat{n} \times \vec{a}_2 \cdot \vec{S}_1 \vec{a}_1 \cdot \vec{v}_2 - \frac{4}{3} \hat{n} \times \vec{S}_1 \cdot \vec{v}_2 \vec{a}_2 \cdot \vec{a}_2 + \frac{8}{3} \hat{n} \times \vec{S}_1 \cdot \vec{v}_2 \vec{a}_2 \cdot \vec{v}_1 - \\
 & \frac{4}{3} \hat{n} \times \vec{S}_1 \cdot \vec{v}_2 \vec{a}_2 \cdot \vec{v}_2 + \frac{4}{3} \hat{n} \times \vec{a}_2 \cdot \vec{S}_1 \vec{a}_2 \cdot \vec{v}_2 - \frac{8}{3} \hat{n} \times \vec{a}_2 \cdot \vec{S}_1 \vec{v}_1 \cdot \vec{v}_2 - \frac{4}{3} \hat{n} \times \vec{S}_1 \cdot \vec{v}_2 \vec{v}_2 \cdot \vec{v}_2 + \frac{4}{3} \hat{n} \times \vec{a}_2 \cdot \vec{S}_1 \vec{v}_2 \cdot \vec{v}_2 \Big) m_2^2 + \\
 & \frac{1}{r^2} G^2 \left( -\frac{28}{3} \hat{n} \times \vec{S}_1 \cdot \vec{v}_2 (\hat{n} \cdot \vec{v}_2)^3 - 16 \hat{n} \times \vec{a}_2 \cdot \vec{S}_1 (\hat{n} \cdot \vec{v}_2)^3 + \frac{8}{3} \vec{S}_1 \times \vec{v}_1 \cdot \vec{v}_2 (\hat{n} \cdot \vec{v}_2)^2 - \frac{4}{3} \vec{a}_1 \times \vec{S}_1 \cdot \vec{v}_2 (\hat{n} \cdot \vec{v}_2)^2 - \right. \\
 & \frac{20}{3} \vec{a}_2 \times \vec{S}_1 \cdot \vec{v}_1 (\hat{n} \cdot \vec{v}_2)^2 + \frac{28}{3} \vec{a}_2 \times \vec{S}_1 \cdot \vec{v}_2 (\hat{n} \cdot \vec{v}_2)^2 + \frac{16}{3} \hat{n} \times \vec{S}_1 \cdot \vec{v}_2 \hat{n} \cdot \vec{a}_1 (\hat{n} \cdot \vec{v}_2)^2 + \\
 & \frac{32}{3} \hat{n} \times \vec{S}_1 \cdot \vec{v}_2 \hat{n} \cdot \vec{a}_2 (\hat{n} \cdot \vec{v}_2)^2 + \frac{32}{3} \hat{n} \times \vec{S}_1 \cdot \vec{v}_2 \hat{n} \cdot \vec{v}_1 (\hat{n} \cdot \vec{v}_2)^2 + \frac{80}{3} \hat{n} \times \vec{a}_2 \cdot \vec{S}_1 \hat{n} \cdot \vec{v}_1 (\hat{n} \cdot \vec{v}_2)^2 - \\
 & \frac{32}{3} \hat{n} \times \vec{a}_2 \cdot \vec{S}_1 (\hat{n} \cdot \vec{v}_1)^2 \hat{n} \cdot \vec{v}_2 - \frac{20}{3} \vec{S}_1 \times \vec{v}_1 \cdot \vec{v}_2 \hat{n} \cdot \vec{a}_2 \hat{n} \cdot \vec{v}_2 + \frac{16}{3} \vec{a}_2 \times \vec{S}_1 \cdot \vec{v}_1 \hat{n} \cdot \vec{v}_1 \hat{n} \cdot \vec{v}_2 - \\
 & \left. \frac{20}{3} \vec{a}_2 \times \vec{S}_1 \cdot \vec{v}_2 \hat{n} \cdot \vec{v}_1 \hat{n} \cdot \vec{v}_2 - \frac{80}{3} \hat{n} \times \vec{S}_1 \cdot \vec{v}_2 \hat{n} \cdot \vec{a}_2 \hat{n} \cdot \vec{v}_1 \hat{n} \cdot \vec{v}_2 - \frac{8}{3} \hat{n} \times \vec{S}_1 \cdot \vec{v}_2 \vec{a}_1 \cdot \vec{v}_2 \hat{n} \cdot \vec{v}_2 + \right.
 \end{aligned}$$

$$\begin{aligned}
& \frac{20}{3} \hat{n} \times \vec{S}_1 \cdot \vec{v}_2 \vec{a}_2 \cdot \vec{v}_1 \hat{n} \cdot \vec{v}_2 - \frac{28}{3} \hat{n} \times \vec{S}_1 \cdot \vec{v}_2 \vec{a}_2 \cdot \vec{v}_2 \hat{n} \cdot \vec{v}_2 + \frac{8}{3} \hat{n} \times \vec{a}_2 \cdot \vec{S}_1 \vec{v}_1 \cdot \vec{v}_1 \hat{n} \cdot \vec{v}_2 - \\
& \frac{16}{3} \hat{n} \times \vec{S}_1 \cdot \vec{v}_2 \vec{v}_1 \cdot \vec{v}_2 \hat{n} \cdot \vec{v}_2 - \frac{40}{3} \hat{n} \times \vec{a}_2 \cdot \vec{S}_1 \vec{v}_1 \cdot \vec{v}_2 \hat{n} \cdot \vec{v}_2 - 2 \hat{n} \times \vec{S}_1 \cdot \vec{v}_2 \vec{v}_2 \cdot \vec{v}_2 \hat{n} \cdot \vec{v}_2 + 8 \hat{n} \times \vec{a}_2 \cdot \vec{S}_1 \vec{v}_2 \cdot \vec{v}_2 \hat{n} \cdot \vec{v}_2 + \\
& \frac{32}{3} \hat{n} \times \vec{S}_1 \cdot \vec{v}_2 \hat{n} \cdot \vec{a}_2 (\hat{n} \cdot \vec{v}_1)^2 + \frac{16}{3} \vec{S}_1 \times \vec{v}_1 \cdot \vec{v}_2 \hat{n} \cdot \vec{a}_2 \hat{n} \cdot \vec{v}_1 - \frac{8}{3} \vec{S}_1 \times \vec{v}_1 \cdot \vec{v}_2 \vec{a}_2 \cdot \vec{v}_1 - \frac{16}{3} \hat{n} \times \vec{S}_1 \cdot \vec{v}_2 \hat{n} \cdot \vec{v}_1 \vec{a}_2 \cdot \vec{v}_1 + \\
& \frac{4}{3} \vec{S}_1 \times \vec{v}_1 \cdot \vec{v}_2 \vec{a}_2 \cdot \vec{v}_2 + \frac{8}{3} \hat{n} \times \vec{S}_1 \cdot \vec{v}_2 \hat{n} \cdot \vec{v}_1 \vec{a}_2 \cdot \vec{v}_2 - \frac{8}{3} \hat{n} \times \vec{S}_1 \cdot \vec{v}_2 \hat{n} \cdot \vec{a}_2 \vec{v}_1 \cdot \vec{v}_1 - \frac{8}{3} \vec{a}_2 \times \vec{S}_1 \cdot \vec{v}_1 \vec{v}_1 \cdot \vec{v}_2 + \\
& \frac{10}{3} \vec{a}_2 \times \vec{S}_1 \cdot \vec{v}_2 \vec{v}_1 \cdot \vec{v}_2 + \frac{20}{3} \hat{n} \times \vec{S}_1 \cdot \vec{v}_2 \hat{n} \cdot \vec{a}_2 \vec{v}_1 \cdot \vec{v}_2 + \frac{16}{3} \hat{n} \times \vec{a}_2 \cdot \vec{S}_1 \hat{n} \cdot \vec{v}_1 \vec{v}_1 \cdot \vec{v}_2 + \frac{8}{3} \vec{S}_1 \times \vec{v}_1 \cdot \vec{v}_2 \vec{v}_2 \cdot \vec{v}_2 - \\
& \frac{4}{3} \vec{a}_1 \times \vec{S}_1 \cdot \vec{v}_2 \vec{v}_2 \cdot \vec{v}_2 + \frac{4}{3} \vec{a}_2 \times \vec{S}_1 \cdot \vec{v}_1 \vec{v}_2 \cdot \vec{v}_2 - \frac{14}{3} \vec{a}_2 \times \vec{S}_1 \cdot \vec{v}_2 \vec{v}_2 \cdot \vec{v}_2 + \frac{8}{3} \hat{n} \times \vec{S}_1 \cdot \vec{v}_2 \hat{n} \cdot \vec{a}_1 \vec{v}_2 \cdot \vec{v}_2 + \\
& \frac{4}{3} \hat{n} \times \vec{S}_1 \cdot \vec{v}_2 \hat{n} \cdot \vec{a}_2 \vec{v}_2 \cdot \vec{v}_2 + \frac{16}{3} \hat{n} \times \vec{S}_1 \cdot \vec{v}_2 \hat{n} \cdot \vec{v}_1 \vec{v}_2 \cdot \vec{v}_2 - \frac{8}{3} \hat{n} \times \vec{a}_2 \cdot \vec{S}_1 \hat{n} \cdot \vec{v}_1 \vec{v}_2 \cdot \vec{v}_2 \Big) m_2^2 + \\
& \frac{1}{r^3} G^2 \left( -24 \hat{n} \times \vec{S}_1 \cdot \vec{v}_2 (\hat{n} \cdot \vec{v}_2)^4 + \frac{28}{3} \vec{S}_1 \times \vec{v}_1 \cdot \vec{v}_2 (\hat{n} \cdot \vec{v}_2)^3 + 56 \hat{n} \times \vec{S}_1 \cdot \vec{v}_2 \hat{n} \cdot \vec{v}_1 (\hat{n} \cdot \vec{v}_2)^3 - \right. \\
& 32 \hat{n} \times \vec{S}_1 \cdot \vec{v}_2 (\hat{n} \cdot \vec{v}_1)^2 (\hat{n} \cdot \vec{v}_2)^2 - \frac{32}{3} \vec{S}_1 \times \vec{v}_1 \cdot \vec{v}_2 \hat{n} \cdot \vec{v}_1 (\hat{n} \cdot \vec{v}_2)^2 + \frac{16}{3} \hat{n} \times \vec{S}_1 \cdot \vec{v}_2 \vec{v}_1 \cdot \vec{v}_1 (\hat{n} \cdot \vec{v}_2)^2 - \\
& 28 \hat{n} \times \vec{S}_1 \cdot \vec{v}_2 \vec{v}_1 \cdot \vec{v}_2 (\hat{n} \cdot \vec{v}_2)^2 + 4 \hat{n} \times \vec{S}_1 \cdot \vec{v}_2 \vec{v}_2 \cdot \vec{v}_2 (\hat{n} \cdot \vec{v}_2)^2 + \frac{16}{3} \vec{S}_1 \times \vec{v}_1 \cdot \vec{v}_2 \vec{v}_1 \cdot \vec{v}_2 \hat{n} \cdot \vec{v}_2 + \\
& \frac{64}{3} \hat{n} \times \vec{S}_1 \cdot \vec{v}_2 \hat{n} \cdot \vec{v}_1 \vec{v}_1 \cdot \vec{v}_2 \hat{n} \cdot \vec{v}_2 + 2 \vec{S}_1 \times \vec{v}_1 \cdot \vec{v}_2 \vec{v}_2 \cdot \vec{v}_2 \hat{n} \cdot \vec{v}_2 + 8 \hat{n} \times \vec{S}_1 \cdot \vec{v}_2 \hat{n} \cdot \vec{v}_1 \vec{v}_2 \cdot \vec{v}_2 \hat{n} \cdot \vec{v}_2 - \\
& \frac{8}{3} \hat{n} \times \vec{S}_1 \cdot \vec{v}_2 (\vec{v}_1 \cdot \vec{v}_2)^2 + 2 \hat{n} \times \vec{S}_1 \cdot \vec{v}_2 (\vec{v}_2 \cdot \vec{v}_2)^2 - \frac{32}{3} \hat{n} \times \vec{S}_1 \cdot \vec{v}_2 (\hat{n} \cdot \vec{v}_1)^2 \vec{v}_2 \cdot \vec{v}_2 - \\
& \left. \frac{16}{3} \vec{S}_1 \times \vec{v}_1 \cdot \vec{v}_2 \hat{n} \cdot \vec{v}_1 \vec{v}_2 \cdot \vec{v}_2 + \frac{8}{3} \hat{n} \times \vec{S}_1 \cdot \vec{v}_2 \vec{v}_1 \cdot \vec{v}_1 \vec{v}_2 \cdot \vec{v}_2 - 2 \hat{n} \times \vec{S}_1 \cdot \vec{v}_2 \vec{v}_1 \cdot \vec{v}_2 \vec{v}_2 \cdot \vec{v}_2 \right) m_2^2 \Big\}
\end{aligned}$$

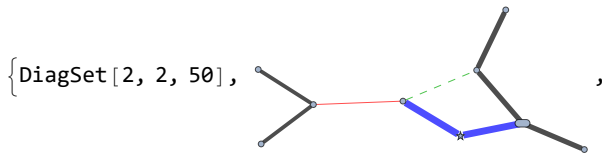

$$\begin{aligned}
& \frac{1}{r} \left( \frac{4}{3} \hat{n} \times \vec{S}_1 \cdot \vec{v}_1 (\hat{n} \cdot \vec{a}_1)^2 + 2 \vec{S}_1 \times \vec{a}_1 \cdot \vec{v}_2 \hat{n} \cdot \vec{a}_1 - 2 \vec{S}_1 \times \vec{v}_1 \cdot \vec{a}_1 \hat{n} \cdot \vec{a}_1 + \frac{2}{3} \vec{S}_1 \times \vec{v}_1 \cdot \vec{a}_2 \hat{n} \cdot \vec{a}_1 - \frac{4}{3} \hat{n} \times \vec{S}_1 \cdot \vec{v}_1 \hat{n} \cdot \vec{a}_2 \hat{n} \cdot \vec{a}_1 + \right. \\
& \frac{4}{3} \hat{n} \times \vec{S}_1 \cdot \vec{v}_1 \hat{n} \cdot \vec{v}_1 \hat{n} \cdot \vec{a}_1 + \frac{8}{3} \hat{n} \times \vec{S}_1 \cdot \vec{a}_1 \hat{n} \cdot \vec{v}_1 \hat{n} \cdot \vec{a}_1 - 4 \hat{n} \times \vec{S}_1 \cdot \vec{a}_1 \hat{n} \cdot \vec{v}_2 \hat{n} \cdot \vec{a}_1 + \frac{8}{3} \hat{n} \times \vec{S}_1 \cdot \vec{a}_1 (\hat{n} \cdot \vec{v}_1)^2 + \\
& \frac{4}{3} \hat{n} \times \vec{S}_1 \cdot \vec{a}_1 (\hat{n} \cdot \vec{v}_1)^2 - \frac{4}{3} \vec{S}_1 \times \vec{v}_1 \cdot \vec{a}_1 \hat{n} \cdot \vec{a}_2 + 2 \vec{S}_1 \times \vec{a}_1 \cdot \vec{v}_2 \hat{n} \cdot \vec{v}_1 + \frac{2}{3} \vec{S}_1 \times \vec{v}_1 \cdot \vec{a}_2 \hat{n} \cdot \vec{v}_1 + \\
& \frac{10}{3} \vec{S}_1 \times \vec{v}_1 \cdot \vec{a}_1 \hat{n} \cdot \vec{v}_1 - \frac{4}{3} \hat{n} \times \vec{S}_1 \cdot \vec{v}_1 \hat{n} \cdot \vec{a}_2 \hat{n} \cdot \vec{v}_1 - 4 \hat{n} \times \vec{S}_1 \cdot \vec{a}_1 \hat{n} \cdot \vec{v}_1 \hat{n} \cdot \vec{v}_2 - \frac{14}{3} \hat{n} \times \vec{S}_1 \cdot \vec{v}_1 \vec{a}_1 \cdot \vec{a}_1 + \\
& \frac{2}{3} \hat{n} \times \vec{S}_1 \cdot \vec{v}_1 \vec{a}_1 \cdot \vec{a}_2 + 2 \hat{n} \times \vec{S}_1 \cdot \vec{a}_1 \vec{a}_1 \cdot \vec{v}_2 + 2 \hat{n} \times \vec{S}_1 \cdot \vec{v}_1 \vec{v}_1 \cdot \vec{a}_1 - \frac{14}{3} \hat{n} \times \vec{S}_1 \cdot \vec{v}_1 \vec{v}_1 \cdot \vec{a}_1 - \frac{10}{3} \hat{n} \times \vec{S}_1 \cdot \vec{a}_1 \vec{v}_1 \cdot \vec{a}_1 + \\
& \left. \frac{2}{3} \hat{n} \times \vec{S}_1 \cdot \vec{v}_1 \vec{v}_1 \cdot \vec{a}_2 - \frac{10}{3} \hat{n} \times \vec{S}_1 \cdot \vec{a}_1 \vec{v}_1 \cdot \vec{v}_1 - \frac{2}{3} \hat{n} \times \vec{S}_1 \cdot \vec{a}_1 \vec{v}_1 \cdot \vec{v}_1 + 2 \hat{n} \times \vec{S}_1 \cdot \vec{a}_1 \vec{v}_1 \cdot \vec{v}_2 \right) m_1 m_2 G^2 + \\
& \frac{1}{r^2} \left( -4 \hat{n} \times \vec{S}_1 \cdot \vec{v}_1 (\hat{n} \cdot \vec{v}_1)^3 - \frac{8}{3} \hat{n} \times \vec{S}_1 \cdot \vec{a}_1 (\hat{n} \cdot \vec{v}_1)^3 - \frac{7}{3} \vec{S}_1 \times \vec{v}_1 \cdot \vec{v}_2 (\hat{n} \cdot \vec{v}_1)^2 - \frac{5}{3} \vec{S}_1 \times \vec{a}_1 \cdot \vec{v}_2 (\hat{n} \cdot \vec{v}_1)^2 - \right. \\
& \frac{17}{3} \vec{S}_1 \times \vec{v}_1 \cdot \vec{a}_1 (\hat{n} \cdot \vec{v}_1)^2 - \frac{1}{3} \vec{S}_1 \times \vec{v}_1 \cdot \vec{a}_2 (\hat{n} \cdot \vec{v}_1)^2 - \frac{16}{3} \hat{n} \times \vec{S}_1 \cdot \vec{v}_1 \hat{n} \cdot \vec{a}_1 (\hat{n} \cdot \vec{v}_1)^2 + \frac{4}{3} \hat{n} \times \vec{S}_1 \cdot \vec{v}_1 \hat{n} \cdot \vec{a}_2 (\hat{n} \cdot \vec{v}_1)^2 + \\
& \frac{28}{3} \hat{n} \times \vec{S}_1 \cdot \vec{v}_1 \hat{n} \cdot \vec{v}_2 (\hat{n} \cdot \vec{v}_1)^2 + \frac{20}{3} \hat{n} \times \vec{S}_1 \cdot \vec{a}_1 \hat{n} \cdot \vec{v}_2 (\hat{n} \cdot \vec{v}_1)^2 - \frac{16}{3} \hat{n} \times \vec{S}_1 \cdot \vec{v}_1 (\hat{n} \cdot \vec{v}_2)^2 \hat{n} \cdot \vec{v}_1 - \\
& \frac{7}{3} \vec{S}_1 \times \vec{v}_1 \cdot \vec{v}_2 \hat{n} \cdot \vec{a}_1 \hat{n} \cdot \vec{v}_1 + \frac{8}{3} \vec{S}_1 \times \vec{v}_1 \cdot \vec{v}_2 \hat{n} \cdot \vec{v}_2 \hat{n} \cdot \vec{v}_1 + 10 \vec{S}_1 \times \vec{v}_1 \cdot \vec{a}_1 \hat{n} \cdot \vec{v}_2 \hat{n} \cdot \vec{v}_1 + \\
& \left. \frac{28}{3} \hat{n} \times \vec{S}_1 \cdot \vec{v}_1 \hat{n} \cdot \vec{a}_1 \hat{n} \cdot \vec{v}_2 \hat{n} \cdot \vec{v}_1 - \frac{7}{3} \hat{n} \times \vec{S}_1 \cdot \vec{v}_1 \vec{a}_1 \cdot \vec{v}_2 \hat{n} \cdot \vec{v}_1 + \frac{11}{3} \hat{n} \times \vec{S}_1 \cdot \vec{v}_1 \vec{v}_1 \cdot \vec{a}_1 \hat{n} \cdot \vec{v}_1 - \right.
\end{aligned}$$

$$\begin{aligned}
& \frac{2}{3} \hat{n} \times \vec{S}_1 \cdot \vec{v}_1 \vec{v}_1 \cdot \vec{a}_2 \hat{n} \cdot \vec{v}_1 + 10 \hat{n} \times \vec{S}_1 \cdot \vec{v}_1 \vec{v}_1 \cdot \vec{v}_1 \hat{n} \cdot \vec{v}_1 + \hat{n} \times \vec{S}_1 \cdot \vec{a}_1 \vec{v}_1 \cdot \vec{v}_1 \hat{n} \cdot \vec{v}_1 - \frac{14}{3} \hat{n} \times \vec{S}_1 \cdot \vec{v}_1 \vec{v}_1 \cdot \vec{v}_2 \hat{n} \cdot \vec{v}_1 - \\
& \frac{10}{3} \hat{n} \times \vec{S}_1 \cdot \vec{a}_1 \vec{v}_1 \cdot \vec{v}_2 \hat{n} \cdot \vec{v}_1 + \frac{4}{3} \hat{n} \times \vec{S}_1 \cdot \vec{v}_1 \vec{v}_2 \cdot \vec{v}_2 \hat{n} \cdot \vec{v}_1 - \frac{8}{3} \vec{S}_1 \times \vec{v}_1 \cdot \vec{a}_1 (\hat{n} \cdot \vec{v}_2)^2 - \frac{16}{3} \hat{n} \times \vec{S}_1 \cdot \vec{v}_1 \hat{n} \cdot \vec{a}_1 (\hat{n} \cdot \vec{v}_2)^2 + \\
& \frac{8}{3} \vec{S}_1 \times \vec{v}_1 \cdot \vec{v}_2 \hat{n} \cdot \vec{a}_1 \hat{n} \cdot \vec{v}_2 - \frac{4}{3} \vec{S}_1 \times \vec{v}_1 \cdot \vec{v}_2 \vec{a}_1 \cdot \vec{v}_2 + \frac{8}{3} \hat{n} \times \vec{S}_1 \cdot \vec{v}_1 \hat{n} \cdot \vec{v}_2 \vec{a}_1 \cdot \vec{v}_2 + \frac{5}{3} \vec{S}_1 \times \vec{v}_1 \cdot \vec{v}_2 \vec{v}_1 \cdot \vec{a}_1 - \\
& \frac{10}{3} \hat{n} \times \vec{S}_1 \cdot \vec{v}_1 \hat{n} \cdot \vec{v}_2 \vec{v}_1 \cdot \vec{a}_1 + \frac{17}{3} \vec{S}_1 \times \vec{v}_1 \cdot \vec{v}_2 \vec{v}_1 \cdot \vec{v}_1 + \frac{1}{3} \vec{S}_1 \times \vec{a}_1 \cdot \vec{v}_2 \vec{v}_1 \cdot \vec{v}_1 + \frac{10}{3} \vec{S}_1 \times \vec{v}_1 \cdot \vec{a}_1 \vec{v}_1 \cdot \vec{v}_1 - \\
& \frac{7}{3} \vec{S}_1 \times \vec{v}_1 \cdot \vec{a}_2 \vec{v}_1 \cdot \vec{v}_1 - \frac{2}{3} \hat{n} \times \vec{S}_1 \cdot \vec{v}_1 \hat{n} \cdot \vec{a}_1 \vec{v}_1 \cdot \vec{v}_1 + \frac{14}{3} \hat{n} \times \vec{S}_1 \cdot \vec{v}_1 \hat{n} \cdot \vec{a}_2 \vec{v}_1 \cdot \vec{v}_1 - \frac{34}{3} \hat{n} \times \vec{S}_1 \cdot \vec{v}_1 \hat{n} \cdot \vec{v}_2 \vec{v}_1 \cdot \vec{v}_1 - \\
& \frac{2}{3} \hat{n} \times \vec{S}_1 \cdot \vec{a}_1 \hat{n} \cdot \vec{v}_2 \vec{v}_1 \cdot \vec{v}_1 - \frac{4}{3} \vec{S}_1 \times \vec{v}_1 \cdot \vec{v}_2 \vec{v}_1 \cdot \vec{v}_2 - 5 \vec{S}_1 \times \vec{v}_1 \cdot \vec{a}_1 \vec{v}_1 \cdot \vec{v}_2 - \frac{7}{3} \hat{n} \times \vec{S}_1 \cdot \vec{v}_1 \hat{n} \cdot \vec{a}_1 \vec{v}_1 \cdot \vec{v}_2 + \\
& \frac{8}{3} \hat{n} \times \vec{S}_1 \cdot \vec{v}_1 \hat{n} \cdot \vec{v}_2 \vec{v}_1 \cdot \vec{v}_2 + \frac{4}{3} \vec{S}_1 \times \vec{v}_1 \cdot \vec{a}_1 \vec{v}_2 \cdot \vec{v}_2 + \frac{4}{3} \hat{n} \times \vec{S}_1 \cdot \vec{v}_1 \hat{n} \cdot \vec{a}_1 \vec{v}_2 \cdot \vec{v}_2 \Big) m_1 m_2 G^2 + \frac{1}{r^3} \\
& \left( 4 \hat{n} \times \vec{S}_1 \cdot \vec{v}_1 (\hat{n} \cdot \vec{v}_1)^4 + 2 \vec{S}_1 \times \vec{v}_1 \cdot \vec{v}_2 (\hat{n} \cdot \vec{v}_1)^3 - 12 \hat{n} \times \vec{S}_1 \cdot \vec{v}_1 \hat{n} \cdot \vec{v}_2 (\hat{n} \cdot \vec{v}_1)^3 + 8 \hat{n} \times \vec{S}_1 \cdot \vec{v}_1 (\hat{n} \cdot \vec{v}_2)^2 (\hat{n} \cdot \vec{v}_1)^2 - \right. \\
& \frac{8}{3} \vec{S}_1 \times \vec{v}_1 \cdot \vec{v}_2 \hat{n} \cdot \vec{v}_2 (\hat{n} \cdot \vec{v}_1)^2 + 4 \hat{n} \times \vec{S}_1 \cdot \vec{v}_1 \vec{v}_1 \cdot \vec{v}_1 (\hat{n} \cdot \vec{v}_1)^2 + 6 \hat{n} \times \vec{S}_1 \cdot \vec{v}_1 \vec{v}_1 \cdot \vec{v}_2 (\hat{n} \cdot \vec{v}_1)^2 - \\
& \frac{4}{3} \hat{n} \times \vec{S}_1 \cdot \vec{v}_1 \vec{v}_2 \cdot \vec{v}_2 (\hat{n} \cdot \vec{v}_1)^2 + 4 \vec{S}_1 \times \vec{v}_1 \cdot \vec{v}_2 \vec{v}_1 \cdot \vec{v}_1 \hat{n} \cdot \vec{v}_1 - 16 \hat{n} \times \vec{S}_1 \cdot \vec{v}_1 \hat{n} \cdot \vec{v}_2 \vec{v}_1 \cdot \vec{v}_1 \hat{n} \cdot \vec{v}_1 + \frac{4}{3} \vec{S}_1 \times \vec{v}_1 \cdot \vec{v}_2 \\
& \vec{v}_1 \cdot \vec{v}_2 \hat{n} \cdot \vec{v}_1 - \frac{16}{3} \hat{n} \times \vec{S}_1 \cdot \vec{v}_1 \hat{n} \cdot \vec{v}_2 \vec{v}_1 \cdot \vec{v}_2 \hat{n} \cdot \vec{v}_1 + \frac{2}{3} \hat{n} \times \vec{S}_1 \cdot \vec{v}_1 (\vec{v}_1 \cdot \vec{v}_2)^2 + \frac{56}{3} \hat{n} \times \vec{S}_1 \cdot \vec{v}_1 (\hat{n} \cdot \vec{v}_2)^2 \vec{v}_1 \cdot \vec{v}_1 - \\
& \left. \frac{28}{3} \vec{S}_1 \times \vec{v}_1 \cdot \vec{v}_2 \hat{n} \cdot \vec{v}_2 \vec{v}_1 \cdot \vec{v}_1 + 4 \hat{n} \times \vec{S}_1 \cdot \vec{v}_1 \vec{v}_1 \cdot \vec{v}_1 \vec{v}_1 \cdot \vec{v}_2 - \frac{14}{3} \hat{n} \times \vec{S}_1 \cdot \vec{v}_1 \vec{v}_1 \cdot \vec{v}_1 \vec{v}_2 \cdot \vec{v}_2 \right) m_1 m_2 G^2 + \\
& m_1 m_2 \left( \frac{4}{3} \log \left( \frac{r}{R_0} \right) \frac{1}{\vec{S}_1 \times \vec{v}_1 \cdot \vec{a}_1} - \frac{2}{9} \frac{1}{\vec{S}_1 \times \vec{v}_1 \cdot \vec{a}_1} - \frac{2}{9} \vec{S}_1 \times \vec{a}_1 \cdot \frac{1}{\vec{a}_1} - \frac{4}{3} \hat{n} \times \vec{S}_1 \cdot \frac{1}{\vec{a}_1} \hat{n} \cdot \vec{a}_1 - \right. \\
& \left. \frac{4}{3} \hat{n} \times \vec{S}_1 \cdot \frac{1}{\vec{a}_1} \hat{n} \cdot \vec{v}_1 + \frac{4}{3} \vec{S}_1 \times \vec{a}_1 \cdot \frac{1}{\vec{a}_1} \log \left( \frac{r}{R_0} \right) + \frac{-\frac{2}{3} \vec{S}_1 \times \vec{v}_1 \cdot \frac{1}{\vec{a}_1} - \frac{2}{3} \vec{S}_1 \times \vec{a}_1 \cdot \frac{1}{\vec{a}_1}}{\epsilon_d} \right) G^2 \Big\}
\end{aligned}$$

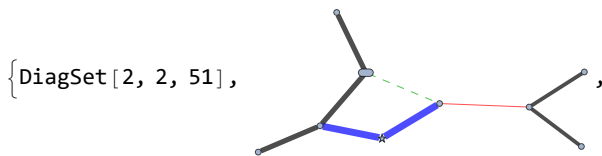

$$\begin{aligned}
& \left( \frac{4}{3} \hat{n} \times \vec{S}_1 \cdot \vec{v}_1 \hat{n} \cdot \vec{a}_1 + \frac{4}{3} \hat{n} \times \vec{S}_1 \cdot \vec{a}_1 \hat{n} \cdot \vec{v}_1 \right) m_1 m_2 G^2 + \frac{1}{r} \left( -4 \hat{n} \times \vec{S}_1 \cdot \vec{v}_1 (\hat{n} \cdot \vec{a}_1)^2 - \frac{10}{3} \vec{S}_1 \times \vec{v}_1 \cdot \vec{v}_2 \hat{n} \cdot \vec{a}_1 - 2 \vec{S}_1 \times \vec{v}_1 \cdot \vec{a}_2 \hat{n} \cdot \vec{a}_1 + \right. \\
& 4 \hat{n} \times \vec{S}_1 \cdot \vec{v}_1 \hat{n} \cdot \vec{a}_2 \hat{n} \cdot \vec{a}_1 - 8 \hat{n} \times \vec{S}_1 \cdot \vec{v}_1 \hat{n} \cdot \vec{v}_1 \hat{n} \cdot \vec{a}_1 - 4 \hat{n} \times \vec{S}_1 \cdot \vec{a}_1 \hat{n} \cdot \vec{v}_1 \hat{n} \cdot \vec{a}_1 + \frac{20}{3} \hat{n} \times \vec{S}_1 \cdot \vec{v}_1 \hat{n} \cdot \vec{v}_2 \hat{n} \cdot \vec{a}_1 - \\
& 8 \hat{n} \times \vec{S}_1 \cdot \vec{a}_1 (\hat{n} \cdot \vec{v}_1)^2 + \frac{4}{3} \hat{n} \times \vec{S}_1 \cdot \vec{v}_1 (\hat{n} \cdot \vec{v}_1)^2 - \frac{10}{3} \vec{S}_1 \times \vec{a}_1 \cdot \vec{v}_2 \hat{n} \cdot \vec{v}_1 - 2 \vec{S}_1 \times \vec{a}_1 \cdot \vec{a}_2 \hat{n} \cdot \vec{v}_1 + 4 \hat{n} \times \vec{S}_1 \cdot \vec{a}_1 \hat{n} \cdot \vec{a}_2 \hat{n} \cdot \vec{v}_1 + \\
& \frac{20}{3} \hat{n} \times \vec{S}_1 \cdot \vec{a}_1 \hat{n} \cdot \vec{v}_1 \hat{n} \cdot \vec{v}_2 + 2 \hat{n} \times \vec{S}_1 \cdot \vec{v}_1 \vec{a}_1 \cdot \vec{a}_1 - 2 \hat{n} \times \vec{S}_1 \cdot \vec{v}_1 \vec{a}_1 \cdot \vec{a}_2 - \frac{10}{3} \hat{n} \times \vec{S}_1 \cdot \vec{v}_1 \vec{a}_1 \cdot \vec{v}_2 + 4 \hat{n} \times \vec{S}_1 \cdot \vec{v}_1 \vec{v}_1 \cdot \vec{a}_1 + \\
& \left. 2 \hat{n} \times \vec{S}_1 \cdot \vec{a}_1 \vec{v}_1 \cdot \vec{a}_1 - 2 \hat{n} \times \vec{S}_1 \cdot \vec{a}_1 \vec{v}_1 \cdot \vec{a}_2 + 4 \hat{n} \times \vec{S}_1 \cdot \vec{a}_1 \vec{v}_1 \cdot \vec{v}_1 - \frac{2}{3} \hat{n} \times \vec{S}_1 \cdot \vec{v}_1 \vec{v}_1 \cdot \vec{v}_1 - \frac{10}{3} \hat{n} \times \vec{S}_1 \cdot \vec{a}_1 \vec{v}_1 \cdot \vec{v}_2 \right) m_1 m_2 G^2 + \\
& \frac{1}{r^2} \left( -8 \hat{n} \times \vec{S}_1 \cdot \vec{v}_1 (\hat{n} \cdot \vec{v}_1)^3 + 20 \hat{n} \times \vec{S}_1 \cdot \vec{a}_1 (\hat{n} \cdot \vec{v}_1)^3 - \frac{7}{3} \vec{S}_1 \times \vec{v}_1 \cdot \vec{v}_2 (\hat{n} \cdot \vec{v}_1)^2 + 9 \vec{S}_1 \times \vec{a}_1 \cdot \vec{v}_2 (\hat{n} \cdot \vec{v}_1)^2 + \right. \\
& 6 \vec{S}_1 \times \vec{v}_1 \cdot \vec{a}_1 (\hat{n} \cdot \vec{v}_1)^2 - \vec{S}_1 \times \vec{v}_1 \cdot \vec{a}_2 (\hat{n} \cdot \vec{v}_1)^2 + 16 \hat{n} \times \vec{S}_1 \cdot \vec{v}_1 \hat{n} \cdot \vec{a}_1 (\hat{n} \cdot \vec{v}_1)^2 + 4 \hat{n} \times \vec{S}_1 \cdot \vec{v}_1 \hat{n} \cdot \vec{a}_2 (\hat{n} \cdot \vec{v}_1)^2 + \\
& \left. \frac{28}{3} \hat{n} \times \vec{S}_1 \cdot \vec{v}_1 \hat{n} \cdot \vec{v}_2 (\hat{n} \cdot \vec{v}_1)^2 - 36 \hat{n} \times \vec{S}_1 \cdot \vec{a}_1 \hat{n} \cdot \vec{v}_2 (\hat{n} \cdot \vec{v}_1)^2 + 16 \hat{n} \times \vec{S}_1 \cdot \vec{a}_1 (\hat{n} \cdot \vec{v}_2)^2 \hat{n} \cdot \vec{v}_1 + \right.
\end{aligned}$$

$$\{\text{DiagSet}[2, 2, 52],$$

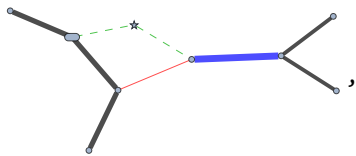

Printed by Wolfram Mathematica Student Edition



$$2 \vec{S}_1 \times \vec{v}_1 \cdot \vec{v}_2 \hat{n} \cdot \vec{v}_2 \vec{v}_1 \cdot \vec{v}_1 - \vec{S}_1 \times \vec{v}_1 \cdot \vec{v}_2 \hat{n} \cdot \vec{v}_2 \vec{v}_1 \cdot \vec{v}_2 + \hat{n} \times \vec{S}_1 \cdot \vec{v}_2 \vec{v}_1 \cdot \vec{v}_1 \vec{v}_2 \cdot \vec{v}_2 \Big) m_1 m_2 G^2 \Big\}$$

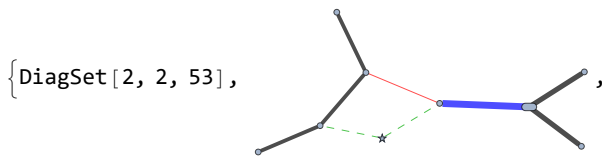

$$\begin{aligned} & \frac{1}{r} G^2 \left( \frac{8}{3} \hat{n} \times \frac{1}{a_2} \cdot \vec{S}_1 (\hat{n} \cdot \vec{v}_1)^2 - \frac{8}{3} \frac{1}{a_2} \times \vec{S}_1 \cdot \vec{v}_1 \hat{n} \cdot \vec{v}_1 + 2 \frac{1}{a_2} \times \vec{S}_1 \cdot \vec{v}_2 \hat{n} \cdot \vec{v}_1 - \frac{4}{3} \hat{n} \times \vec{S}_1 \cdot \vec{v}_2 \hat{n} \cdot \vec{a}_2 \hat{n} \cdot \vec{v}_1 - \right. \\ & \quad \frac{4}{3} \hat{n} \times \vec{a}_2 \cdot \vec{S}_1 \hat{n} \cdot \vec{a}_2 \hat{n} \cdot \vec{v}_1 - 4 \hat{n} \times \frac{1}{a_2} \cdot \vec{S}_1 \hat{n} \cdot \vec{v}_2 \hat{n} \cdot \vec{v}_1 + \frac{4}{3} \hat{n} \times \vec{a}_2 \cdot \vec{S}_1 \hat{n} \cdot \vec{v}_2 \hat{n} \cdot \vec{v}_1 - \frac{2}{3} \frac{1}{S_1} \times \vec{v}_1 \cdot \vec{v}_2 \hat{n} \cdot \vec{a}_2 + \\ & \quad \frac{2}{3} \vec{a}_1 \times \vec{S}_1 \cdot \vec{v}_2 \hat{n} \cdot \vec{a}_2 + \frac{2}{3} \vec{a}_2 \times \vec{S}_1 \cdot \vec{v}_1 \hat{n} \cdot \vec{a}_2 - \frac{4}{3} \hat{n} \times \vec{S}_1 \cdot \vec{v}_2 \hat{n} \cdot \vec{a}_1 \hat{n} \cdot \vec{a}_2 + 2 \frac{1}{a_2} \times \vec{S}_1 \cdot \vec{v}_1 \hat{n} \cdot \vec{v}_2 - \frac{2}{3} \vec{a}_1 \times \vec{a}_2 \cdot \vec{S}_1 \hat{n} \cdot \vec{v}_2 - \\ & \quad \frac{2}{3} \vec{a}_2 \times \vec{S}_1 \cdot \vec{v}_1 \hat{n} \cdot \vec{v}_2 + \frac{4}{3} \hat{n} \times \vec{a}_2 \cdot \vec{S}_1 \hat{n} \cdot \vec{a}_1 \hat{n} \cdot \vec{v}_2 + 2 \hat{n} \times \vec{S}_1 \cdot \vec{v}_2 \frac{1}{a_2} \cdot \vec{v}_1 - \frac{10}{3} \hat{n} \times \vec{S}_1 \cdot \vec{v}_2 \vec{a}_1 \cdot \vec{a}_2 + \frac{10}{3} \hat{n} \times \vec{a}_2 \cdot \vec{S}_1 \vec{a}_1 \cdot \vec{v}_2 - \\ & \quad \left. \frac{10}{3} \hat{n} \times \vec{S}_1 \cdot \vec{v}_2 \vec{a}_2 \cdot \vec{v}_1 - \frac{10}{3} \hat{n} \times \vec{a}_2 \cdot \vec{S}_1 \vec{a}_2 \cdot \vec{v}_1 - \frac{4}{3} \hat{n} \times \frac{1}{a_2} \cdot \vec{S}_1 \vec{v}_1 \cdot \vec{v}_1 + \frac{10}{3} \hat{n} \times \vec{a}_2 \cdot \vec{S}_1 \vec{v}_1 \cdot \vec{v}_2 \right) m_2^2 + \\ & \frac{1}{r^2} G^2 \left( \frac{16}{3} \hat{n} \times \vec{S}_1 \cdot \vec{v}_2 \hat{n} \cdot \vec{a}_2 (\hat{n} \cdot \vec{v}_1)^2 - \frac{16}{3} \hat{n} \times \vec{a}_2 \cdot \vec{S}_1 \hat{n} \cdot \vec{v}_2 (\hat{n} \cdot \vec{v}_1)^2 + 4 \hat{n} \times \vec{a}_2 \cdot \vec{S}_1 (\hat{n} \cdot \vec{v}_2)^2 \hat{n} \cdot \vec{v}_1 + \right. \\ & \quad \frac{8}{3} \vec{S}_1 \times \vec{v}_1 \cdot \vec{v}_2 \hat{n} \cdot \vec{a}_2 \hat{n} \cdot \vec{v}_1 + \frac{8}{3} \vec{a}_2 \times \vec{S}_1 \cdot \vec{v}_1 \hat{n} \cdot \vec{v}_2 \hat{n} \cdot \vec{v}_1 - \frac{4}{3} \vec{a}_2 \times \vec{S}_1 \cdot \vec{v}_2 \hat{n} \cdot \vec{v}_2 \hat{n} \cdot \vec{v}_1 - \\ & \quad \frac{8}{3} \hat{n} \times \vec{S}_1 \cdot \vec{v}_2 \hat{n} \cdot \vec{a}_2 \hat{n} \cdot \vec{v}_2 \hat{n} \cdot \vec{v}_1 + \frac{16}{3} \hat{n} \times \vec{S}_1 \cdot \vec{v}_2 \vec{a}_2 \cdot \vec{v}_1 \hat{n} \cdot \vec{v}_1 - \frac{4}{3} \hat{n} \times \vec{S}_1 \cdot \vec{v}_2 \vec{a}_2 \cdot \vec{v}_2 \hat{n} \cdot \vec{v}_1 - \\ & \quad \frac{16}{3} \hat{n} \times \vec{a}_2 \cdot \vec{S}_1 \vec{v}_1 \cdot \vec{v}_2 \hat{n} \cdot \vec{v}_1 + 4 \hat{n} \times \vec{S}_1 \cdot \vec{v}_2 \vec{v}_2 \cdot \vec{v}_2 \hat{n} \cdot \vec{v}_1 + 6 \hat{n} \times \vec{a}_2 \cdot \vec{S}_1 \vec{v}_2 \cdot \vec{v}_2 \hat{n} \cdot \vec{v}_1 - \vec{a}_2 \times \vec{S}_1 \cdot \vec{v}_1 (\hat{n} \cdot \vec{v}_2)^2 - \\ & \quad \frac{2}{3} \vec{S}_1 \times \vec{v}_1 \cdot \vec{v}_2 \hat{n} \cdot \vec{a}_2 \hat{n} \cdot \vec{v}_2 - 8 \hat{n} \times \vec{S}_1 \cdot \vec{v}_2 \hat{n} \cdot \vec{v}_2 \vec{a}_1 \cdot \vec{v}_2 + \frac{8}{3} \vec{S}_1 \times \vec{v}_1 \cdot \vec{v}_2 \vec{a}_2 \cdot \vec{v}_1 + \frac{2}{3} \hat{n} \times \vec{S}_1 \cdot \vec{v}_2 \hat{n} \cdot \vec{v}_2 \vec{a}_2 \cdot \vec{v}_1 - \\ & \quad \frac{2}{3} \vec{S}_1 \times \vec{v}_1 \cdot \vec{v}_2 \vec{a}_2 \cdot \vec{v}_2 - \frac{4}{3} \hat{n} \times \vec{S}_1 \cdot \vec{v}_2 \hat{n} \cdot \vec{a}_2 \vec{v}_1 \cdot \vec{v}_1 + \frac{4}{3} \hat{n} \times \vec{a}_2 \cdot \vec{S}_1 \hat{n} \cdot \vec{v}_2 \vec{v}_1 \cdot \vec{v}_1 + \frac{8}{3} \vec{a}_2 \times \vec{S}_1 \cdot \vec{v}_1 \vec{v}_1 \cdot \vec{v}_2 + \\ & \quad \frac{8}{3} \vec{a}_2 \times \vec{S}_1 \cdot \vec{v}_2 \vec{v}_1 \cdot \vec{v}_2 - \frac{10}{3} \hat{n} \times \vec{S}_1 \cdot \vec{v}_2 \hat{n} \cdot \vec{a}_2 \vec{v}_1 \cdot \vec{v}_2 - 8 \hat{n} \times \vec{S}_1 \cdot \vec{v}_2 \hat{n} \cdot \vec{v}_2 \vec{v}_1 \cdot \vec{v}_2 - 2 \hat{n} \times \vec{a}_2 \cdot \vec{S}_1 \hat{n} \cdot \vec{v}_2 \vec{v}_1 \cdot \vec{v}_2 + \\ & \quad \left. 2 \vec{S}_1 \times \vec{v}_1 \cdot \vec{v}_2 \vec{v}_2 \cdot \vec{v}_2 - 2 \vec{a}_1 \times \vec{S}_1 \cdot \vec{v}_2 \vec{v}_2 \cdot \vec{v}_2 - 3 \vec{a}_2 \times \vec{S}_1 \cdot \vec{v}_1 \vec{v}_2 \cdot \vec{v}_2 + 4 \hat{n} \times \vec{S}_1 \cdot \vec{v}_2 \hat{n} \cdot \vec{a}_1 \vec{v}_2 \cdot \vec{v}_2 \right) m_2^2 + \\ & \frac{1}{r^3} G^2 \left( -16 \hat{n} \times \vec{S}_1 \cdot \vec{v}_2 \vec{v}_2 \cdot \vec{v}_2 (\hat{n} \cdot \vec{v}_1)^2 + 32 \hat{n} \times \vec{S}_1 \cdot \vec{v}_2 \hat{n} \cdot \vec{v}_2 \vec{v}_1 \cdot \vec{v}_2 \hat{n} \cdot \vec{v}_1 - 8 \vec{S}_1 \times \vec{v}_1 \cdot \vec{v}_2 \vec{v}_2 \cdot \vec{v}_2 \hat{n} \cdot \vec{v}_1 + \right. \\ & \quad 8 \hat{n} \times \vec{S}_1 \cdot \vec{v}_2 \hat{n} \cdot \vec{v}_2 \vec{v}_2 \cdot \vec{v}_2 \hat{n} \cdot \vec{v}_1 - 8 \hat{n} \times \vec{S}_1 \cdot \vec{v}_2 (\vec{v}_1 \cdot \vec{v}_2)^2 - 16 \hat{n} \times \vec{S}_1 \cdot \vec{v}_2 (\hat{n} \cdot \vec{v}_2)^2 \vec{v}_1 \cdot \vec{v}_2 + \\ & \quad \left. 8 \vec{S}_1 \times \vec{v}_1 \cdot \vec{v}_2 \hat{n} \cdot \vec{v}_2 \vec{v}_1 \cdot \vec{v}_2 + 2 \vec{S}_1 \times \vec{v}_1 \cdot \vec{v}_2 \hat{n} \cdot \vec{v}_2 \vec{v}_2 \cdot \vec{v}_2 + 4 \hat{n} \times \vec{S}_1 \cdot \vec{v}_2 \vec{v}_1 \cdot \vec{v}_1 \vec{v}_2 \cdot \vec{v}_2 + 2 \hat{n} \times \vec{S}_1 \cdot \vec{v}_2 \vec{v}_1 \cdot \vec{v}_2 \vec{v}_2 \cdot \vec{v}_2 \right) m_2^2 + \\ & G^2 \left( -\frac{4}{3} \log\left(\frac{r}{R_\theta}\right) \frac{1}{a_2} \times \vec{S}_1 \cdot \vec{v}_1 + \frac{14}{9} \frac{1}{a_2} \times \vec{S}_1 \cdot \vec{v}_1 + \frac{14}{9} \vec{a}_1 \times \frac{1}{a_2} \cdot \vec{S}_1 - \frac{4}{3} \hat{n} \times \frac{1}{a_2} \cdot \vec{S}_1 \hat{n} \cdot \vec{a}_1 - \right. \\ & \quad \left. \frac{4}{3} \hat{n} \times \frac{1}{a_2} \cdot \vec{S}_1 \hat{n} \cdot \vec{v}_1 - \frac{4}{3} \vec{a}_1 \times \frac{1}{a_2} \cdot \vec{S}_1 \log\left(\frac{r}{R_\theta}\right) + \frac{\frac{2}{3} \frac{1}{a_2} \times \vec{S}_1 \cdot \vec{v}_1 + \frac{2}{3} \vec{a}_1 \times \frac{1}{a_2} \cdot \vec{S}_1}{\epsilon_d} \right) m_2^2 \Big\} \end{aligned}$$

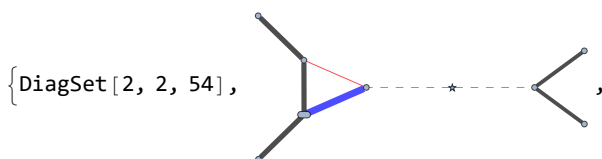

$$\frac{1}{r} \left( -\frac{2}{3} \hat{n} \times \vec{S}_1 \cdot \vec{a}_2 (\hat{n} \cdot \vec{v}_1)^2 - \frac{2}{3} \hat{n} \times \vec{S}_1 \cdot \frac{1}{a_2} (\hat{n} \cdot \vec{v}_1)^2 - \frac{5}{3} \frac{1}{S_1} \times \vec{v}_1 \cdot \vec{a}_2 \hat{n} \cdot \vec{v}_1 + \frac{1}{3} \frac{1}{S_1} \times \vec{v}_2 \cdot \vec{a}_2 \hat{n} \cdot \vec{v}_1 - \frac{5}{3} \vec{S}_1 \times \vec{a}_1 \cdot \vec{a}_2 \hat{n} \cdot \vec{v}_1 - \right.$$



{DiagSet[2, 2, 55],

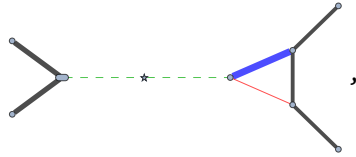

,

$$\begin{aligned}
 & G^2 \left( \frac{4}{3} \hat{n} \times \vec{a}_2 \cdot \vec{S}_1 \hat{n} \cdot \vec{v}_2 - \frac{4}{3} \hat{n} \times \vec{S}_1 \cdot \vec{v}_2 \hat{n} \cdot \vec{a}_2 \right) m_2^2 + \frac{1}{r} G^2 \left( -\frac{8}{3} \hat{n} \times \vec{S}_1 \cdot \vec{v}_2 (\hat{n} \cdot \vec{v}_2)^2 + \frac{8}{3} \hat{n} \times \vec{a}_2 \cdot \vec{S}_1 (\hat{n} \cdot \vec{v}_2)^2 + \right. \\
 & \quad \frac{4}{3} \vec{a}_1 \times \vec{a}_2 \cdot \vec{S}_1 \hat{n} \cdot \vec{v}_2 + \frac{8}{3} \vec{a}_2 \times \vec{S}_1 \cdot \vec{v}_1 \hat{n} \cdot \vec{v}_2 - \frac{8}{3} \hat{n} \times \vec{a}_2 \cdot \vec{S}_1 \hat{n} \cdot \vec{a}_1 \hat{n} \cdot \vec{v}_2 - \frac{16}{3} \hat{n} \times \vec{S}_1 \cdot \vec{v}_2 \hat{n} \cdot \vec{a}_2 \hat{n} \cdot \vec{v}_2 - \\
 & \quad \frac{16}{3} \hat{n} \times \vec{a}_2 \cdot \vec{S}_1 \hat{n} \cdot \vec{v}_1 \hat{n} \cdot \vec{v}_2 + \frac{8}{3} \vec{S}_1 \times \vec{v}_1 \cdot \vec{v}_2 \hat{n} \cdot \vec{a}_2 - \frac{4}{3} \vec{a}_1 \times \vec{S}_1 \cdot \vec{v}_2 \hat{n} \cdot \vec{a}_2 + \frac{8}{3} \hat{n} \times \vec{S}_1 \cdot \vec{v}_2 \hat{n} \cdot \vec{a}_1 \hat{n} \cdot \vec{a}_2 + \\
 & \quad \frac{16}{3} \hat{n} \times \vec{S}_1 \cdot \vec{v}_2 \hat{n} \cdot \vec{a}_2 \hat{n} \cdot \vec{v}_1 - \frac{4}{3} \hat{n} \times \vec{S}_1 \cdot \vec{v}_2 \vec{a}_1 \cdot \vec{a}_2 + \frac{4}{3} \hat{n} \times \vec{a}_2 \cdot \vec{S}_1 \vec{a}_1 \cdot \vec{v}_2 - \frac{8}{3} \hat{n} \times \vec{S}_1 \cdot \vec{v}_2 \vec{a}_2 \cdot \vec{v}_1 + \\
 & \quad \left. \frac{8}{3} \hat{n} \times \vec{S}_1 \cdot \vec{v}_2 \vec{a}_2 \cdot \vec{v}_2 + \frac{8}{3} \hat{n} \times \vec{a}_2 \cdot \vec{S}_1 \vec{v}_1 \cdot \vec{v}_2 + \frac{4}{3} \hat{n} \times \vec{S}_1 \cdot \vec{v}_2 \vec{v}_2 \cdot \vec{v}_2 - \frac{4}{3} \hat{n} \times \vec{a}_2 \cdot \vec{S}_1 \vec{v}_2 \cdot \vec{v}_2 \right) m_2^2 + \frac{1}{r^2} \\
 & G^2 \left( -\frac{32}{3} \hat{n} \times \vec{S}_1 \cdot \vec{v}_2 (\hat{n} \cdot \vec{v}_2)^3 + \frac{16}{3} \vec{S}_1 \times \vec{v}_1 \cdot \vec{v}_2 (\hat{n} \cdot \vec{v}_2)^2 - \frac{8}{3} \vec{a}_1 \times \vec{S}_1 \cdot \vec{v}_2 (\hat{n} \cdot \vec{v}_2)^2 + \frac{8}{3} \vec{a}_2 \times \vec{S}_1 \cdot \vec{v}_1 (\hat{n} \cdot \vec{v}_2)^2 + \right. \\
 & \quad \frac{32}{3} \hat{n} \times \vec{S}_1 \cdot \vec{v}_2 \hat{n} \cdot \vec{a}_1 (\hat{n} \cdot \vec{v}_2)^2 + \frac{64}{3} \hat{n} \times \vec{S}_1 \cdot \vec{v}_2 \hat{n} \cdot \vec{v}_1 (\hat{n} \cdot \vec{v}_2)^2 - \frac{32}{3} \hat{n} \times \vec{a}_2 \cdot \vec{S}_1 \hat{n} \cdot \vec{v}_1 (\hat{n} \cdot \vec{v}_2)^2 + \\
 & \quad \frac{32}{3} \hat{n} \times \vec{a}_2 \cdot \vec{S}_1 (\hat{n} \cdot \vec{v}_1)^2 \hat{n} \cdot \vec{v}_2 + \frac{16}{3} \vec{S}_1 \times \vec{v}_1 \cdot \vec{v}_2 \hat{n} \cdot \vec{a}_2 \hat{n} \cdot \vec{v}_2 - \frac{16}{3} \vec{a}_2 \times \vec{S}_1 \cdot \vec{v}_1 \hat{n} \cdot \vec{v}_1 \hat{n} \cdot \vec{v}_2 + \\
 & \quad \frac{64}{3} \hat{n} \times \vec{S}_1 \cdot \vec{v}_2 \hat{n} \cdot \vec{a}_2 \hat{n} \cdot \vec{v}_1 \hat{n} \cdot \vec{v}_2 - \frac{16}{3} \hat{n} \times \vec{S}_1 \cdot \vec{v}_2 \vec{a}_1 \cdot \vec{v}_2 \hat{n} \cdot \vec{v}_2 - \frac{16}{3} \hat{n} \times \vec{S}_1 \cdot \vec{v}_2 \vec{a}_2 \cdot \vec{v}_1 \hat{n} \cdot \vec{v}_2 - \\
 & \quad \frac{8}{3} \hat{n} \times \vec{a}_2 \cdot \vec{S}_1 \vec{v}_1 \cdot \vec{v}_1 \hat{n} \cdot \vec{v}_2 - \frac{32}{3} \hat{n} \times \vec{S}_1 \cdot \vec{v}_2 \vec{v}_1 \cdot \vec{v}_2 \hat{n} \cdot \vec{v}_2 + \frac{16}{3} \hat{n} \times \vec{a}_2 \cdot \vec{S}_1 \vec{v}_1 \cdot \vec{v}_2 \hat{n} \cdot \vec{v}_2 + 8 \hat{n} \times \vec{S}_1 \cdot \vec{v}_2 \vec{v}_2 \cdot \vec{v}_2 \hat{n} \cdot \vec{v}_2 - \\
 & \quad \frac{32}{3} \hat{n} \times \vec{S}_1 \cdot \vec{v}_2 \hat{n} \cdot \vec{a}_2 (\hat{n} \cdot \vec{v}_1)^2 - \frac{16}{3} \vec{S}_1 \times \vec{v}_1 \cdot \vec{v}_2 \hat{n} \cdot \vec{a}_2 \hat{n} \cdot \vec{v}_1 + \frac{8}{3} \vec{S}_1 \times \vec{v}_1 \cdot \vec{v}_2 \vec{a}_2 \cdot \vec{v}_1 + \frac{16}{3} \hat{n} \times \vec{S}_1 \cdot \vec{v}_2 \hat{n} \cdot \vec{v}_1 \vec{a}_2 \cdot \vec{v}_1 - \\
 & \quad \frac{8}{3} \vec{S}_1 \times \vec{v}_1 \cdot \vec{v}_2 \vec{a}_2 \cdot \vec{v}_2 - \frac{16}{3} \hat{n} \times \vec{S}_1 \cdot \vec{v}_2 \hat{n} \cdot \vec{v}_1 \vec{a}_2 \cdot \vec{v}_2 + \frac{8}{3} \hat{n} \times \vec{S}_1 \cdot \vec{v}_2 \hat{n} \cdot \vec{a}_2 \vec{v}_1 \cdot \vec{v}_1 + \frac{8}{3} \vec{a}_2 \times \vec{S}_1 \cdot \vec{v}_1 \vec{v}_1 \cdot \vec{v}_2 - \\
 & \quad \frac{16}{3} \hat{n} \times \vec{S}_1 \cdot \vec{v}_2 \hat{n} \cdot \vec{a}_2 \vec{v}_1 \cdot \vec{v}_2 - \frac{16}{3} \hat{n} \times \vec{a}_2 \cdot \vec{S}_1 \hat{n} \cdot \vec{v}_1 \vec{v}_1 \cdot \vec{v}_2 - \frac{8}{3} \vec{S}_1 \times \vec{v}_1 \cdot \vec{v}_2 \vec{v}_2 \cdot \vec{v}_2 + \frac{4}{3} \vec{a}_1 \times \vec{S}_1 \cdot \vec{v}_2 \vec{v}_2 \cdot \vec{v}_2 - \\
 & \quad \left. \frac{4}{3} \vec{a}_2 \times \vec{S}_1 \cdot \vec{v}_1 \vec{v}_2 \cdot \vec{v}_2 - \frac{8}{3} \hat{n} \times \vec{S}_1 \cdot \vec{v}_2 \hat{n} \cdot \vec{a}_1 \vec{v}_2 \cdot \vec{v}_2 - \frac{16}{3} \hat{n} \times \vec{S}_1 \cdot \vec{v}_2 \hat{n} \cdot \vec{v}_1 \vec{v}_2 \cdot \vec{v}_2 + \frac{8}{3} \hat{n} \times \vec{a}_2 \cdot \vec{S}_1 \hat{n} \cdot \vec{v}_1 \vec{v}_2 \cdot \vec{v}_2 \right) m_2^2 + \\
 & \quad \frac{1}{r^3} G^2 \left( \frac{32}{3} \vec{S}_1 \times \vec{v}_1 \cdot \vec{v}_2 (\hat{n} \cdot \vec{v}_2)^3 + 64 \hat{n} \times \vec{S}_1 \cdot \vec{v}_2 \hat{n} \cdot \vec{v}_1 (\hat{n} \cdot \vec{v}_2)^3 - 64 \hat{n} \times \vec{S}_1 \cdot \vec{v}_2 (\hat{n} \cdot \vec{v}_1)^2 (\hat{n} \cdot \vec{v}_2)^2 - \right. \\
 & \quad \frac{64}{3} \vec{S}_1 \times \vec{v}_1 \cdot \vec{v}_2 \hat{n} \cdot \vec{v}_1 (\hat{n} \cdot \vec{v}_2)^2 + \frac{32}{3} \hat{n} \times \vec{S}_1 \cdot \vec{v}_2 \vec{v}_1 \cdot \vec{v}_1 (\hat{n} \cdot \vec{v}_2)^2 - 32 \hat{n} \times \vec{S}_1 \cdot \vec{v}_2 \vec{v}_1 \cdot \vec{v}_2 (\hat{n} \cdot \vec{v}_2)^2 + \\
 & \quad \frac{32}{3} \vec{S}_1 \times \vec{v}_1 \cdot \vec{v}_2 \vec{v}_1 \cdot \vec{v}_2 \hat{n} \cdot \vec{v}_2 + \frac{128}{3} \hat{n} \times \vec{S}_1 \cdot \vec{v}_2 \hat{n} \cdot \vec{v}_1 \vec{v}_1 \cdot \vec{v}_2 \hat{n} \cdot \vec{v}_2 - 8 \vec{S}_1 \times \vec{v}_1 \cdot \vec{v}_2 \vec{v}_2 \cdot \vec{v}_2 \hat{n} \cdot \vec{v}_2 - \\
 & \quad 32 \hat{n} \times \vec{S}_1 \cdot \vec{v}_2 \hat{n} \cdot \vec{v}_1 \vec{v}_2 \cdot \vec{v}_2 \hat{n} \cdot \vec{v}_2 - \frac{16}{3} \hat{n} \times \vec{S}_1 \cdot \vec{v}_2 (\vec{v}_1 \cdot \vec{v}_2)^2 + \frac{32}{3} \hat{n} \times \vec{S}_1 \cdot \vec{v}_2 (\hat{n} \cdot \vec{v}_1)^2 \vec{v}_2 \cdot \vec{v}_2 + \\
 & \quad \left. \frac{16}{3} \vec{S}_1 \times \vec{v}_1 \cdot \vec{v}_2 \hat{n} \cdot \vec{v}_1 \vec{v}_2 \cdot \vec{v}_2 - \frac{8}{3} \hat{n} \times \vec{S}_1 \cdot \vec{v}_2 \vec{v}_1 \cdot \vec{v}_1 \vec{v}_2 \cdot \vec{v}_2 + 8 \hat{n} \times \vec{S}_1 \cdot \vec{v}_2 \vec{v}_1 \cdot \vec{v}_2 \vec{v}_2 \cdot \vec{v}_2 \right) m_2^2 \Big\}
 \end{aligned}$$

{DiagSet[2, 2, 56],

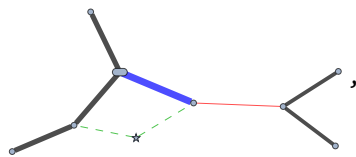

,

$$\begin{aligned}
 & \frac{1}{r} \left( \frac{4}{3} \hat{n} \times \vec{S}_1 \cdot \vec{v}_1 (\hat{n} \cdot \vec{a}_1)^2 + \frac{2}{3} \vec{S}_1 \times \vec{a}_1 \cdot \vec{v}_2 \hat{n} \cdot \vec{a}_1 - 2 \vec{S}_1 \times \vec{v}_1 \cdot \vec{a}_1 \hat{n} \cdot \vec{a}_1 + \frac{4}{3} \hat{n} \times \vec{S}_1 \cdot \vec{v}_1 \hat{n} \cdot \vec{v}_1 \hat{n} \cdot \vec{a}_1 + \frac{8}{3} \hat{n} \times \vec{S}_1 \cdot \vec{a}_1 \hat{n} \cdot \vec{v}_1 \hat{n} \cdot \vec{a}_1 - \right. \\
 & \quad \left. \frac{4}{3} \hat{n} \times \vec{S}_1 \cdot \vec{a}_1 \hat{n} \cdot \vec{v}_2 \hat{n} \cdot \vec{a}_1 + \frac{8}{3} \hat{n} \times \vec{S}_1 \cdot \vec{a}_1 (\hat{n} \cdot \vec{v}_1)^2 - 4 \hat{n} \times \vec{S}_1 \cdot \vec{a}_1 (\hat{n} \cdot \vec{v}_1)^2 + \frac{4}{3} \vec{S}_1 \times \vec{v}_1 \cdot \vec{a}_1 \hat{n} \cdot \vec{a}_2 + \frac{2}{3} \vec{S}_1 \times \vec{a}_1 \cdot \vec{v}_2 \hat{n} \cdot \vec{v}_1 - \right.
 \end{aligned}$$

$$\begin{aligned}
& \frac{4}{3} \vec{S}_1 \times \vec{a}_1 \cdot \vec{v}_2 \hat{n} \cdot \vec{v}_1 + \frac{2}{3} \vec{S}_1 \times \vec{a}_1 \cdot \vec{a}_2 \hat{n} \cdot \vec{v}_1 - 2 \vec{S}_1 \times \vec{v}_1 \cdot \vec{a}_1 \hat{n} \cdot \vec{v}_1 - \frac{4}{3} \hat{n} \times \vec{S}_1 \cdot \vec{a}_1 \hat{n} \cdot \vec{a}_2 \hat{n} \cdot \vec{v}_1 + \frac{4}{3} \vec{S}_1 \times \vec{v}_1 \cdot \vec{a}_1 \hat{n} \cdot \vec{v}_2 + \\
& \frac{4}{3} \vec{S}_1 \times \vec{v}_1 \cdot \vec{a}_1 \hat{n} \cdot \vec{v}_2 - \frac{4}{3} \hat{n} \times \vec{S}_1 \cdot \vec{a}_1 \hat{n} \cdot \vec{v}_1 \hat{n} \cdot \vec{v}_2 + \frac{8}{3} \hat{n} \times \vec{S}_1 \cdot \vec{a}_1 \hat{n} \cdot \vec{v}_1 \hat{n} \cdot \vec{v}_2 - \frac{14}{3} \hat{n} \times \vec{S}_1 \cdot \vec{v}_1 \vec{a}_1 \cdot \vec{a}_1 + \\
& \frac{2}{3} \hat{n} \times \vec{S}_1 \cdot \vec{a}_1 \vec{a}_1 \cdot \vec{v}_2 + 2 \hat{n} \times \vec{S}_1 \cdot \vec{v}_1 \vec{v}_1 \cdot \vec{a}_1 - \frac{14}{3} \hat{n} \times \vec{S}_1 \cdot \vec{v}_1 \vec{v}_1 \cdot \vec{a}_1 - \frac{10}{3} \hat{n} \times \vec{S}_1 \cdot \vec{a}_1 \vec{v}_1 \cdot \vec{a}_1 + \frac{2}{3} \hat{n} \times \vec{S}_1 \cdot \vec{a}_1 \vec{v}_1 \cdot \vec{a}_2 - \\
& \frac{10}{3} \hat{n} \times \vec{S}_1 \cdot \vec{a}_1 \vec{v}_1 \cdot \vec{v}_1 + 2 \hat{n} \times \vec{S}_1 \cdot \vec{a}_1 \vec{v}_1 \cdot \vec{v}_1 + \frac{2}{3} \hat{n} \times \vec{S}_1 \cdot \vec{a}_1 \vec{v}_1 \cdot \vec{v}_2 - \frac{4}{3} \hat{n} \times \vec{S}_1 \cdot \vec{a}_1 \vec{v}_1 \cdot \vec{v}_2 \Big) m_1 m_2 G^2 + \frac{1}{r^2} \\
& \left( -\frac{4}{3} \hat{n} \times \vec{S}_1 \cdot \vec{v}_1 (\hat{n} \cdot \vec{v}_1)^3 - 8 \hat{n} \times \vec{S}_1 \cdot \vec{a}_1 (\hat{n} \cdot \vec{v}_1)^3 - \frac{1}{3} \vec{S}_1 \times \vec{v}_1 \cdot \vec{v}_2 (\hat{n} \cdot \vec{v}_1)^2 - \frac{11}{3} \vec{S}_1 \times \vec{a}_1 \cdot \vec{v}_2 (\hat{n} \cdot \vec{v}_1)^2 - \right. \\
& \frac{11}{3} \vec{S}_1 \times \vec{v}_1 \cdot \vec{a}_1 (\hat{n} \cdot \vec{v}_1)^2 - \frac{1}{3} \vec{S}_1 \times \vec{v}_1 \cdot \vec{a}_2 (\hat{n} \cdot \vec{v}_1)^2 - \frac{16}{3} \hat{n} \times \vec{S}_1 \cdot \vec{v}_1 \hat{n} \cdot \vec{a}_1 (\hat{n} \cdot \vec{v}_1)^2 + \frac{4}{3} \hat{n} \times \vec{S}_1 \cdot \vec{v}_1 \hat{n} \cdot \vec{a}_2 (\hat{n} \cdot \vec{v}_1)^2 + \\
& \frac{4}{3} \hat{n} \times \vec{S}_1 \cdot \vec{v}_1 \hat{n} \cdot \vec{v}_2 (\hat{n} \cdot \vec{v}_1)^2 + \frac{44}{3} \hat{n} \times \vec{S}_1 \cdot \vec{a}_1 \hat{n} \cdot \vec{v}_2 (\hat{n} \cdot \vec{v}_1)^2 - \frac{16}{3} \hat{n} \times \vec{S}_1 \cdot \vec{a}_1 (\hat{n} \cdot \vec{v}_2)^2 \hat{n} \cdot \vec{v}_1 - \\
& \frac{5}{3} \vec{S}_1 \times \vec{v}_1 \cdot \vec{v}_2 \hat{n} \cdot \vec{a}_1 \hat{n} \cdot \vec{v}_1 + \frac{8}{3} \vec{S}_1 \times \vec{a}_1 \cdot \vec{v}_2 \hat{n} \cdot \vec{v}_2 \hat{n} \cdot \vec{v}_1 + \frac{2}{3} \vec{S}_1 \times \vec{v}_1 \cdot \vec{a}_1 \hat{n} \cdot \vec{v}_2 \hat{n} \cdot \vec{v}_1 + \frac{20}{3} \hat{n} \times \vec{S}_1 \cdot \vec{v}_1 \hat{n} \cdot \vec{a}_1 \hat{n} \cdot \vec{v}_2 \hat{n} \cdot \vec{v}_1 - \\
& \frac{5}{3} \hat{n} \times \vec{S}_1 \cdot \vec{v}_1 \vec{a}_1 \cdot \vec{v}_2 \hat{n} \cdot \vec{v}_1 + \frac{17}{3} \hat{n} \times \vec{S}_1 \cdot \vec{v}_1 \vec{v}_1 \cdot \vec{a}_1 \hat{n} \cdot \vec{v}_1 - \frac{2}{3} \hat{n} \times \vec{S}_1 \cdot \vec{v}_1 \vec{v}_1 \cdot \vec{a}_2 \hat{n} \cdot \vec{v}_1 + 6 \hat{n} \times \vec{S}_1 \cdot \vec{v}_1 \vec{v}_1 \cdot \vec{v}_1 \hat{n} \cdot \vec{v}_1 + \\
& 3 \hat{n} \times \vec{S}_1 \cdot \vec{a}_1 \vec{v}_1 \cdot \vec{v}_1 \hat{n} \cdot \vec{v}_1 - \frac{2}{3} \hat{n} \times \vec{S}_1 \cdot \vec{v}_1 \vec{v}_1 \cdot \vec{v}_2 \hat{n} \cdot \vec{v}_1 - \frac{22}{3} \hat{n} \times \vec{S}_1 \cdot \vec{a}_1 \vec{v}_1 \cdot \vec{v}_2 \hat{n} \cdot \vec{v}_1 + \frac{4}{3} \hat{n} \times \vec{S}_1 \cdot \vec{a}_1 \vec{v}_2 \cdot \vec{v}_2 \hat{n} \cdot \vec{v}_1 + \\
& \frac{8}{3} \vec{S}_1 \times \vec{v}_1 \cdot \vec{a}_1 (\hat{n} \cdot \vec{v}_2)^2 + \frac{19}{3} \vec{S}_1 \times \vec{v}_1 \cdot \vec{v}_2 \vec{v}_1 \cdot \vec{a}_1 - \frac{38}{3} \hat{n} \times \vec{S}_1 \cdot \vec{v}_1 \hat{n} \cdot \vec{v}_2 \vec{v}_1 \cdot \vec{a}_1 + \frac{11}{3} \vec{S}_1 \times \vec{v}_1 \cdot \vec{v}_2 \vec{v}_1 \cdot \vec{v}_1 + \\
& \frac{7}{3} \vec{S}_1 \times \vec{a}_1 \cdot \vec{v}_2 \vec{v}_1 \cdot \vec{v}_1 - \frac{2}{3} \vec{S}_1 \times \vec{v}_1 \cdot \vec{a}_1 \vec{v}_1 \cdot \vec{v}_1 + \frac{11}{3} \vec{S}_1 \times \vec{v}_1 \cdot \vec{a}_2 \vec{v}_1 \cdot \vec{v}_1 + \frac{10}{3} \hat{n} \times \vec{S}_1 \cdot \vec{v}_1 \hat{n} \cdot \vec{a}_1 \vec{v}_1 \cdot \vec{v}_1 - \\
& \frac{22}{3} \hat{n} \times \vec{S}_1 \cdot \vec{v}_1 \hat{n} \cdot \vec{a}_2 \vec{v}_1 \cdot \vec{v}_1 - \frac{22}{3} \hat{n} \times \vec{S}_1 \cdot \vec{v}_1 \hat{n} \cdot \vec{v}_2 \vec{v}_1 \cdot \vec{v}_1 - \frac{14}{3} \hat{n} \times \vec{S}_1 \cdot \vec{a}_1 \hat{n} \cdot \vec{v}_2 \vec{v}_1 \cdot \vec{v}_1 - \frac{4}{3} \vec{S}_1 \times \vec{a}_1 \cdot \vec{v}_2 \vec{v}_1 \cdot \vec{v}_2 - \\
& \frac{1}{3} \vec{S}_1 \times \vec{v}_1 \cdot \vec{a}_1 \vec{v}_1 \cdot \vec{v}_2 - \frac{5}{3} \hat{n} \times \vec{S}_1 \cdot \vec{v}_1 \hat{n} \cdot \vec{a}_1 \vec{v}_1 \cdot \vec{v}_2 + \frac{8}{3} \hat{n} \times \vec{S}_1 \cdot \vec{a}_1 \hat{n} \cdot \vec{v}_2 \vec{v}_1 \cdot \vec{v}_2 - \frac{4}{3} \vec{S}_1 \times \vec{v}_1 \cdot \vec{a}_1 \vec{v}_2 \cdot \vec{v}_2 \Big) m_1 m_2 G^2 + \\
& \frac{1}{r^3} \left( 4 \hat{n} \times \vec{S}_1 \cdot \vec{v}_1 (\hat{n} \cdot \vec{v}_1)^4 + 2 \vec{S}_1 \times \vec{v}_1 \cdot \vec{v}_2 (\hat{n} \cdot \vec{v}_1)^3 - 12 \hat{n} \times \vec{S}_1 \cdot \vec{v}_1 \hat{n} \cdot \vec{v}_2 (\hat{n} \cdot \vec{v}_1)^3 + \right. \\
& 8 \hat{n} \times \vec{S}_1 \cdot \vec{v}_1 (\hat{n} \cdot \vec{v}_2)^2 (\hat{n} \cdot \vec{v}_1)^2 - \frac{8}{3} \vec{S}_1 \times \vec{v}_1 \cdot \vec{v}_2 \hat{n} \cdot \vec{v}_2 (\hat{n} \cdot \vec{v}_1)^2 - 12 \hat{n} \times \vec{S}_1 \cdot \vec{v}_1 \vec{v}_1 \cdot \vec{v}_1 (\hat{n} \cdot \vec{v}_1)^2 + \\
& 6 \hat{n} \times \vec{S}_1 \cdot \vec{v}_1 \vec{v}_1 \cdot \vec{v}_2 (\hat{n} \cdot \vec{v}_1)^2 - \frac{4}{3} \hat{n} \times \vec{S}_1 \cdot \vec{v}_1 \vec{v}_2 \cdot \vec{v}_2 (\hat{n} \cdot \vec{v}_1)^2 - 10 \vec{S}_1 \times \vec{v}_1 \cdot \vec{v}_2 \vec{v}_1 \cdot \vec{v}_1 \hat{n} \cdot \vec{v}_1 + \\
& 40 \hat{n} \times \vec{S}_1 \cdot \vec{v}_1 \hat{n} \cdot \vec{v}_2 \vec{v}_1 \cdot \vec{v}_1 \hat{n} \cdot \vec{v}_1 + \frac{4}{3} \vec{S}_1 \times \vec{v}_1 \cdot \vec{v}_2 \vec{v}_1 \cdot \vec{v}_2 \hat{n} \cdot \vec{v}_1 - \frac{16}{3} \hat{n} \times \vec{S}_1 \cdot \vec{v}_1 \hat{n} \cdot \vec{v}_2 \vec{v}_1 \cdot \vec{v}_2 \hat{n} \cdot \vec{v}_1 + \\
& 4 \hat{n} \times \vec{S}_1 \cdot \vec{v}_1 (\vec{v}_1 \cdot \vec{v}_1)^2 + \frac{2}{3} \hat{n} \times \vec{S}_1 \cdot \vec{v}_1 (\vec{v}_1 \cdot \vec{v}_2)^2 - \frac{88}{3} \hat{n} \times \vec{S}_1 \cdot \vec{v}_1 (\hat{n} \cdot \vec{v}_2)^2 \vec{v}_1 \cdot \vec{v}_1 + \\
& \left. \frac{44}{3} \vec{S}_1 \times \vec{v}_1 \cdot \vec{v}_2 \hat{n} \cdot \vec{v}_2 \vec{v}_1 \cdot \vec{v}_1 - 10 \hat{n} \times \vec{S}_1 \cdot \vec{v}_1 \vec{v}_1 \cdot \vec{v}_1 \vec{v}_1 \cdot \vec{v}_2 + \frac{22}{3} \hat{n} \times \vec{S}_1 \cdot \vec{v}_1 \vec{v}_1 \cdot \vec{v}_1 \vec{v}_2 \cdot \vec{v}_2 \right) m_1 m_2 G^2 + \\
& m_1 m_2 \left( -\frac{4}{3} \log\left(\frac{r}{R_\theta}\right) \vec{S}_1 \times \vec{v}_1 \cdot \vec{a}_1 + \frac{14}{9} \vec{S}_1 \times \vec{v}_1 \cdot \vec{a}_1 + \frac{14}{9} \vec{S}_1 \times \vec{a}_1 \cdot \vec{a}_1 + \frac{4}{3} \hat{n} \times \vec{S}_1 \cdot \vec{a}_1 \hat{n} \cdot \vec{a}_1 + \right. \\
& \left. \frac{4}{3} \hat{n} \times \vec{S}_1 \cdot \vec{a}_1 \hat{n} \cdot \vec{v}_1 - \frac{4}{3} \vec{S}_1 \times \vec{a}_1 \cdot \vec{a}_1 \log\left(\frac{r}{R_\theta}\right) + \frac{\frac{2}{3} \vec{S}_1 \times \vec{v}_1 \cdot \vec{a}_1 + \frac{2}{3} \vec{S}_1 \times \vec{a}_1 \cdot \vec{a}_1}{\epsilon_d} \right) G^2 \Big\}
\end{aligned}$$

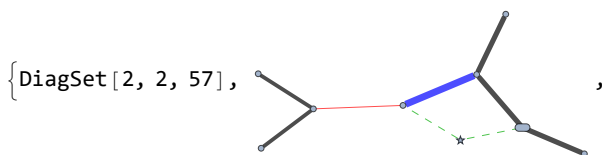

[illegible]

$$\{\text{DiagSet}[2, 2, 58],$$
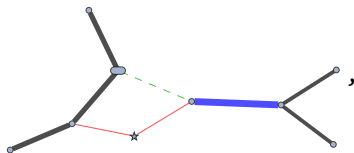

$$\frac{1}{r} \left( \frac{1}{3} \vec{S}_1 \times \vec{v}_1 \cdot \vec{v}_2 \hat{n} \cdot \vec{a}_2 - \vec{S}_1 \times \vec{a}_1 \cdot \vec{v}_2 \hat{n} \cdot \vec{a}_2 + \hat{n} \times \vec{S}_1 \cdot \vec{v}_2 \hat{n} \cdot \vec{a}_1 \hat{n} \cdot \vec{a}_2 - \frac{1}{3} \hat{n} \times \vec{S}_1 \cdot \vec{v}_2 \hat{n} \cdot \vec{v}_1 \hat{n} \cdot \vec{a}_2 - \vec{S}_1 \times \vec{a}_1 \cdot \vec{v}_2 \hat{n} \cdot \vec{v}_2 + \right. \\ \left. \frac{1}{3} \vec{S}_1 \times \vec{v}_1 \cdot \vec{a}_2 \hat{n} \cdot \vec{v}_2 + \frac{1}{3} \vec{S}_1 \times \vec{v}_1 \cdot \vec{v}_2 \hat{n} \cdot \vec{v}_2 - \vec{S}_1 \times \vec{a}_1 \cdot \vec{a}_2 \hat{n} \cdot \vec{v}_2 + \hat{n} \times \vec{S}_1 \cdot \vec{v}_2 \hat{n} \cdot \vec{a}_1 \hat{n} \cdot \vec{v}_2 + \hat{n} \times \vec{S}_1 \cdot \vec{a}_2 \hat{n} \cdot \vec{a}_1 \hat{n} \cdot \vec{v}_2 - \right. \\ \left. \frac{1}{3} \hat{n} \times \vec{S}_1 \cdot \vec{a}_2 \hat{n} \cdot \vec{v}_1 \hat{n} \cdot \vec{v}_2 - \frac{1}{3} \hat{n} \times \vec{S}_1 \cdot \vec{v}_2 \hat{n} \cdot \vec{v}_1 \hat{n} \cdot \vec{v}_2 + \hat{n} \times \vec{S}_1 \cdot \vec{v}_2 \vec{a}_1 \cdot \vec{a}_2 + \hat{n} \times \vec{S}_1 \cdot \vec{v}_2 \vec{a}_1 \cdot \vec{v}_2 + \right. \\ \left. \hat{n} \times \vec{S}_1 \cdot \vec{a}_2 \vec{a}_1 \cdot \vec{v}_2 + \frac{5}{3} \hat{n} \times \vec{S}_1 \cdot \vec{v}_2 \vec{v}_1 \cdot \vec{a}_2 + \frac{5}{3} \hat{n} \times \vec{S}_1 \cdot \vec{a}_2 \vec{v}_1 \cdot \vec{v}_2 + \frac{5}{3} \hat{n} \times \vec{S}_1 \cdot \vec{v}_2 \vec{v}_1 \cdot \vec{v}_2 \right) m_1 m_2 G^2 + \frac{1}{r^2}$$

$$\frac{1}{r^3}$$

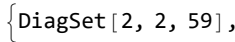

$$\frac{1}{r^2}$$

$$\begin{aligned} & 2 \vec{S}_1 \times \vec{v}_1 \cdot \vec{v}_2 \vec{v}_2 \cdot \vec{v}_2 + 2 \vec{a}_1 \times \vec{S}_1 \cdot \vec{v}_2 \vec{v}_2 \cdot \vec{v}_2 - \frac{7}{3} \vec{a}_2 \times \vec{S}_1 \cdot \vec{v}_1 \vec{v}_2 \cdot \vec{v}_2 - 4 \hat{n} \times \vec{S}_1 \cdot \vec{v}_2 \hat{n} \cdot \vec{a}_1 \vec{v}_2 \cdot \vec{v}_2 \Big) m_2^2 + \\ & \frac{1}{r^3} G^2 \Big( 16 \hat{n} \times \vec{S}_1 \cdot \vec{v}_2 \vec{v}_2 \cdot \vec{v}_2 (\hat{n} \cdot \vec{v}_1)^2 - 32 \hat{n} \times \vec{S}_1 \cdot \vec{v}_2 \hat{n} \cdot \vec{v}_2 \vec{v}_1 \cdot \vec{v}_2 \hat{n} \cdot \vec{v}_1 + 8 \vec{S}_1 \times \vec{v}_1 \cdot \vec{v}_2 \vec{v}_2 \cdot \vec{v}_2 \hat{n} \cdot \vec{v}_1 - \\ & 8 \hat{n} \times \vec{S}_1 \cdot \vec{v}_2 \hat{n} \cdot \vec{v}_2 \vec{v}_2 \cdot \vec{v}_2 \hat{n} \cdot \vec{v}_1 + 8 \hat{n} \times \vec{S}_1 \cdot \vec{v}_2 (\vec{v}_1 \cdot \vec{v}_2)^2 + 16 \hat{n} \times \vec{S}_1 \cdot \vec{v}_2 (\hat{n} \cdot \vec{v}_2)^2 \vec{v}_1 \cdot \vec{v}_2 - \\ & 8 \vec{S}_1 \times \vec{v}_1 \cdot \vec{v}_2 \hat{n} \cdot \vec{v}_2 \vec{v}_1 \cdot \vec{v}_2 - 2 \vec{S}_1 \times \vec{v}_1 \cdot \vec{v}_2 \hat{n} \cdot \vec{v}_2 \vec{v}_2 \cdot \vec{v}_2 - 4 \hat{n} \times \vec{S}_1 \cdot \vec{v}_2 \vec{v}_1 \cdot \vec{v}_1 \vec{v}_2 \cdot \vec{v}_2 - 2 \hat{n} \times \vec{S}_1 \cdot \vec{v}_2 \vec{v}_1 \cdot \vec{v}_2 \vec{v}_2 \cdot \vec{v}_2 \Big) m_2^2 \Big\} \end{aligned}$$

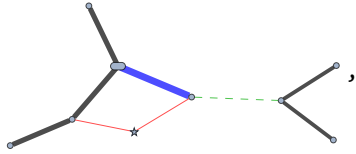

[illegible]

$$\begin{aligned}
& 16 \hat{n} \times \vec{S}_1 \cdot \vec{v}_1 \hat{n} \cdot \vec{v}_2 \vec{v}_1 \cdot \vec{v}_2 \hat{n} \cdot \vec{v}_1 + \frac{16}{3} \hat{n} \times \vec{S}_1 \cdot \vec{v}_2 \hat{n} \cdot \vec{v}_2 \vec{v}_1 \cdot \vec{v}_2 \hat{n} \cdot \vec{v}_1 - \frac{4}{3} \vec{S}_1 \times \vec{v}_1 \cdot \vec{v}_2 \vec{v}_2 \cdot \vec{v}_2 \hat{n} \cdot \vec{v}_1 - \\
& 2 \hat{n} \times \vec{S}_1 \cdot \vec{v}_2 (\vec{v}_1 \cdot \vec{v}_1)^2 + 4 \hat{n} \times \vec{S}_1 \cdot \vec{v}_1 (\vec{v}_1 \cdot \vec{v}_2)^2 - \frac{2}{3} \hat{n} \times \vec{S}_1 \cdot \vec{v}_2 (\vec{v}_1 \cdot \vec{v}_2)^2 + \frac{40}{3} \hat{n} \times \vec{S}_1 \cdot \vec{v}_2 (\hat{n} \cdot \vec{v}_2)^2 \vec{v}_1 \cdot \vec{v}_1 - \\
& 2 \vec{S}_1 \times \vec{v}_1 \cdot \vec{v}_2 \hat{n} \cdot \vec{v}_2 \vec{v}_1 \cdot \vec{v}_1 + 16 \hat{n} \times \vec{S}_1 \cdot \vec{v}_1 (\hat{n} \cdot \vec{v}_2)^2 \vec{v}_1 \cdot \vec{v}_2 - \frac{32}{3} \vec{S}_1 \times \vec{v}_1 \cdot \vec{v}_2 \hat{n} \cdot \vec{v}_2 \vec{v}_1 \cdot \vec{v}_2 - 2 \hat{n} \times \vec{S}_1 \cdot \vec{v}_1 \vec{v}_1 \cdot \vec{v}_1 \vec{v}_1 \cdot \vec{v}_2 + \\
& 6 \hat{n} \times \vec{S}_1 \cdot \vec{v}_2 \vec{v}_1 \cdot \vec{v}_1 \vec{v}_1 \cdot \vec{v}_2 - \frac{10}{3} \hat{n} \times \vec{S}_1 \cdot \vec{v}_2 \vec{v}_1 \cdot \vec{v}_1 \vec{v}_2 \cdot \vec{v}_2 - 4 \hat{n} \times \vec{S}_1 \cdot \vec{v}_1 \vec{v}_1 \cdot \vec{v}_2 \vec{v}_2 \cdot \vec{v}_2 \Big) m_1 m_2 G^2 \Big\}
\end{aligned}$$

{DiagSet[2, 2, 61],

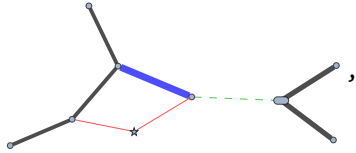

$$\begin{aligned}
& \frac{1}{r} G^2 \left( -\frac{8}{3} \hat{n} \times \vec{S}_1 \cdot \vec{v}_2 (\hat{n} \cdot \vec{a}_2)^2 + \frac{4}{3} \vec{a}_2 \times \vec{S}_1 \cdot \vec{v}_2 \hat{n} \cdot \vec{a}_2 - 4 \hat{n} \times \vec{S}_1 \cdot \vec{v}_2 \hat{n} \cdot \vec{v}_2 \hat{n} \cdot \vec{a}_2 + \frac{8}{3} \hat{n} \times \vec{a}_2 \cdot \vec{S}_1 \hat{n} \cdot \vec{v}_2 \hat{n} \cdot \vec{a}_2 - \right. \\
& \frac{4}{3} \hat{n} \times \vec{S}_1 \cdot \vec{v}_2 (\hat{n} \cdot \vec{v}_2)^2 + \frac{4}{3} \hat{n} \times \vec{a}_2 \cdot \vec{S}_1 (\hat{n} \cdot \vec{v}_2)^2 + \frac{2}{3} \vec{a}_2 \times \vec{S}_1 \cdot \vec{v}_2 \hat{n} \cdot \vec{v}_2 + \frac{4}{3} \hat{n} \times \vec{S}_1 \cdot \vec{v}_2 \vec{a}_2 \cdot \vec{a}_2 + \\
& \left. 4 \hat{n} \times \vec{S}_1 \cdot \vec{v}_2 \vec{a}_2 \cdot \vec{v}_2 - \frac{4}{3} \hat{n} \times \vec{a}_2 \cdot \vec{S}_1 \vec{a}_2 \cdot \vec{v}_2 + \frac{8}{3} \hat{n} \times \vec{S}_1 \cdot \vec{v}_2 \vec{v}_2 \cdot \vec{v}_2 - \frac{8}{3} \hat{n} \times \vec{a}_2 \cdot \vec{S}_1 \vec{v}_2 \cdot \vec{v}_2 \right) m_2^2 + \frac{1}{r^2} \\
& G^2 \left( -\frac{20}{3} \hat{n} \times \vec{S}_1 \cdot \vec{v}_2 (\hat{n} \cdot \vec{v}_2)^3 + \frac{16}{3} \hat{n} \times \vec{a}_2 \cdot \vec{S}_1 (\hat{n} \cdot \vec{v}_2)^3 + \frac{8}{3} \vec{S}_1 \times \vec{v}_1 \cdot \vec{v}_2 (\hat{n} \cdot \vec{v}_2)^2 - \frac{4}{3} \vec{a}_1 \times \vec{S}_1 \cdot \vec{v}_2 (\hat{n} \cdot \vec{v}_2)^2 + \right. \\
& \frac{4}{3} \vec{a}_2 \times \vec{S}_1 \cdot \vec{v}_1 (\hat{n} \cdot \vec{v}_2)^2 - \frac{4}{3} \vec{a}_2 \times \vec{S}_1 \cdot \vec{v}_2 (\hat{n} \cdot \vec{v}_2)^2 + \frac{16}{3} \hat{n} \times \vec{S}_1 \cdot \vec{v}_2 \hat{n} \cdot \vec{a}_1 (\hat{n} \cdot \vec{v}_2)^2 - \frac{32}{3} \hat{n} \times \vec{S}_1 \cdot \vec{v}_2 \hat{n} \cdot \vec{a}_2 (\hat{n} \cdot \vec{v}_2)^2 + \\
& \frac{32}{3} \hat{n} \times \vec{S}_1 \cdot \vec{v}_2 \hat{n} \cdot \vec{v}_1 (\hat{n} \cdot \vec{v}_2)^2 - \frac{16}{3} \hat{n} \times \vec{a}_2 \cdot \vec{S}_1 \hat{n} \cdot \vec{v}_1 (\hat{n} \cdot \vec{v}_2)^2 + 4 \vec{S}_1 \times \vec{v}_1 \cdot \vec{v}_2 \hat{n} \cdot \vec{a}_2 \hat{n} \cdot \vec{v}_2 - \frac{4}{3} \vec{a}_2 \times \vec{S}_1 \cdot \vec{v}_2 \hat{n} \cdot \vec{v}_1 \hat{n} \cdot \vec{v}_2 + \\
& 16 \hat{n} \times \vec{S}_1 \cdot \vec{v}_2 \hat{n} \cdot \vec{a}_2 \hat{n} \cdot \vec{v}_1 \hat{n} \cdot \vec{v}_2 - \frac{8}{3} \hat{n} \times \vec{S}_1 \cdot \vec{v}_2 \vec{a}_1 \cdot \vec{v}_2 \hat{n} \cdot \vec{v}_2 - 4 \hat{n} \times \vec{S}_1 \cdot \vec{v}_2 \vec{a}_2 \cdot \vec{v}_1 \hat{n} \cdot \vec{v}_2 + \frac{4}{3} \hat{n} \times \vec{S}_1 \cdot \vec{v}_2 \vec{a}_2 \cdot \vec{v}_2 \hat{n} \cdot \vec{v}_2 - \\
& \frac{16}{3} \hat{n} \times \vec{S}_1 \cdot \vec{v}_2 \vec{v}_1 \cdot \vec{v}_2 \hat{n} \cdot \vec{v}_2 + \frac{8}{3} \hat{n} \times \vec{a}_2 \cdot \vec{S}_1 \vec{v}_1 \cdot \vec{v}_2 \hat{n} \cdot \vec{v}_2 + 10 \hat{n} \times \vec{S}_1 \cdot \vec{v}_2 \vec{v}_2 \cdot \vec{v}_2 \hat{n} \cdot \vec{v}_2 - 8 \hat{n} \times \vec{a}_2 \cdot \vec{S}_1 \vec{v}_2 \cdot \vec{v}_2 \hat{n} \cdot \vec{v}_2 - \\
& 4 \vec{S}_1 \times \vec{v}_1 \cdot \vec{v}_2 \vec{a}_2 \cdot \vec{v}_2 - 8 \hat{n} \times \vec{S}_1 \cdot \vec{v}_2 \hat{n} \cdot \vec{v}_1 \vec{a}_2 \cdot \vec{v}_2 + \frac{2}{3} \vec{a}_2 \times \vec{S}_1 \cdot \vec{v}_2 \vec{v}_1 \cdot \vec{v}_2 - 4 \hat{n} \times \vec{S}_1 \cdot \vec{v}_2 \hat{n} \cdot \vec{a}_2 \vec{v}_1 \cdot \vec{v}_2 - \\
& \frac{16}{3} \vec{S}_1 \times \vec{v}_1 \cdot \vec{v}_2 \vec{v}_2 \cdot \vec{v}_2 + \frac{8}{3} \vec{a}_1 \times \vec{S}_1 \cdot \vec{v}_2 \vec{v}_2 \cdot \vec{v}_2 - \frac{8}{3} \vec{a}_2 \times \vec{S}_1 \cdot \vec{v}_1 \vec{v}_2 \cdot \vec{v}_2 + \frac{2}{3} \vec{a}_2 \times \vec{S}_1 \cdot \vec{v}_2 \vec{v}_2 \cdot \vec{v}_2 - \\
& \left. \frac{16}{3} \hat{n} \times \vec{S}_1 \cdot \vec{v}_2 \hat{n} \cdot \vec{a}_1 \vec{v}_2 \cdot \vec{v}_2 + \frac{20}{3} \hat{n} \times \vec{S}_1 \cdot \vec{v}_2 \hat{n} \cdot \vec{a}_2 \vec{v}_2 \cdot \vec{v}_2 - \frac{32}{3} \hat{n} \times \vec{S}_1 \cdot \vec{v}_2 \hat{n} \cdot \vec{v}_1 \vec{v}_2 \cdot \vec{v}_2 + \frac{16}{3} \hat{n} \times \vec{a}_2 \cdot \vec{S}_1 \hat{n} \cdot \vec{v}_1 \vec{v}_2 \cdot \vec{v}_2 \right) \\
& m_2^2 + \frac{1}{r^3} G^2 \left( -8 \hat{n} \times \vec{S}_1 \cdot \vec{v}_2 (\hat{n} \cdot \vec{v}_2)^4 + \frac{20}{3} \vec{S}_1 \times \vec{v}_1 \cdot \vec{v}_2 (\hat{n} \cdot \vec{v}_2)^3 + 40 \hat{n} \times \vec{S}_1 \cdot \vec{v}_2 \hat{n} \cdot \vec{v}_1 (\hat{n} \cdot \vec{v}_2)^3 - \right. \\
& 32 \hat{n} \times \vec{S}_1 \cdot \vec{v}_2 (\hat{n} \cdot \vec{v}_1)^2 (\hat{n} \cdot \vec{v}_2)^2 - \frac{32}{3} \vec{S}_1 \times \vec{v}_1 \cdot \vec{v}_2 \hat{n} \cdot \vec{v}_1 (\hat{n} \cdot \vec{v}_2)^2 + \frac{16}{3} \hat{n} \times \vec{S}_1 \cdot \vec{v}_2 \vec{v}_1 \cdot \vec{v}_1 (\hat{n} \cdot \vec{v}_2)^2 - \\
& 20 \hat{n} \times \vec{S}_1 \cdot \vec{v}_2 \vec{v}_1 \cdot \vec{v}_2 (\hat{n} \cdot \vec{v}_2)^2 + 12 \hat{n} \times \vec{S}_1 \cdot \vec{v}_2 \vec{v}_2 \cdot \vec{v}_2 (\hat{n} \cdot \vec{v}_2)^2 + \frac{16}{3} \vec{S}_1 \times \vec{v}_1 \cdot \vec{v}_2 \vec{v}_1 \cdot \vec{v}_2 \hat{n} \cdot \vec{v}_2 + \\
& \frac{64}{3} \hat{n} \times \vec{S}_1 \cdot \vec{v}_2 \hat{n} \cdot \vec{v}_1 \vec{v}_1 \cdot \vec{v}_2 \hat{n} \cdot \vec{v}_2 - 10 \vec{S}_1 \times \vec{v}_1 \cdot \vec{v}_2 \vec{v}_2 \cdot \vec{v}_2 \hat{n} \cdot \vec{v}_2 - 40 \hat{n} \times \vec{S}_1 \cdot \vec{v}_2 \hat{n} \cdot \vec{v}_1 \vec{v}_2 \cdot \vec{v}_2 \hat{n} \cdot \vec{v}_2 - \\
& \frac{8}{3} \hat{n} \times \vec{S}_1 \cdot \vec{v}_2 (\vec{v}_1 \cdot \vec{v}_2)^2 - 2 \hat{n} \times \vec{S}_1 \cdot \vec{v}_2 (\vec{v}_2 \cdot \vec{v}_2)^2 + \frac{64}{3} \hat{n} \times \vec{S}_1 \cdot \vec{v}_2 (\hat{n} \cdot \vec{v}_1)^2 \vec{v}_2 \cdot \vec{v}_2 + \\
& \left. \frac{32}{3} \vec{S}_1 \times \vec{v}_1 \cdot \vec{v}_2 \hat{n} \cdot \vec{v}_1 \vec{v}_2 \cdot \vec{v}_2 - \frac{16}{3} \hat{n} \times \vec{S}_1 \cdot \vec{v}_2 \vec{v}_1 \cdot \vec{v}_1 \vec{v}_2 \cdot \vec{v}_2 + 10 \hat{n} \times \vec{S}_1 \cdot \vec{v}_2 \vec{v}_1 \cdot \vec{v}_2 \vec{v}_2 \cdot \vec{v}_2 \right) m_2^2 \Big\}
\end{aligned}$$

{DiagSet[2, 2, 62],

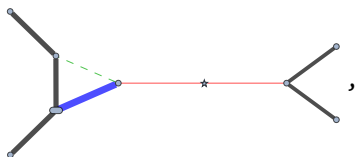



[illegible]

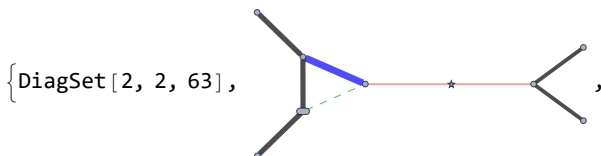

$$\begin{aligned} & \frac{1}{r} \left( \frac{4}{3} \vec{S}_1 \times \vec{v}_1 \cdot \vec{v}_2 \hat{n} \cdot \vec{a}_1 + \vec{S}_1 \times \vec{v}_1 \cdot \vec{a}_2 \hat{n} \cdot \vec{a}_1 - 2 \hat{n} \times \vec{S}_1 \cdot \vec{v}_1 \hat{n} \cdot \vec{a}_2 \hat{n} \cdot \vec{a}_1 - \frac{8}{3} \hat{n} \times \vec{S}_1 \cdot \vec{v}_1 \hat{n} \cdot \vec{v}_2 \hat{n} \cdot \vec{a}_1 + \frac{4}{3} \vec{S}_1 \times \vec{a}_1 \cdot \vec{v}_2 \hat{n} \cdot \vec{v}_1 + \right. \\ & \quad \vec{S}_1 \times \vec{v}_1 \cdot \vec{a}_2 \hat{n} \cdot \vec{v}_1 + \frac{4}{3} \vec{S}_1 \times \vec{v}_1 \cdot \vec{v}_2 \hat{n} \cdot \vec{v}_1 + \vec{S}_1 \times \vec{a}_1 \cdot \vec{a}_2 \hat{n} \cdot \vec{v}_1 - 2 \hat{n} \times \vec{S}_1 \cdot \vec{v}_1 \hat{n} \cdot \vec{a}_2 \hat{n} \cdot \vec{v}_1 - 2 \hat{n} \times \vec{S}_1 \cdot \vec{a}_1 \hat{n} \cdot \vec{a}_2 \hat{n} \cdot \vec{v}_1 - \\ & \quad \frac{8}{3} \hat{n} \times \vec{S}_1 \cdot \vec{a}_1 \hat{n} \cdot \vec{v}_1 \hat{n} \cdot \vec{v}_2 - \frac{8}{3} \hat{n} \times \vec{S}_1 \cdot \vec{v}_1 \hat{n} \cdot \vec{v}_1 \hat{n} \cdot \vec{v}_2 + \hat{n} \times \vec{S}_1 \cdot \vec{v}_1 \vec{a}_1 \cdot \vec{a}_2 + \frac{4}{3} \hat{n} \times \vec{S}_1 \cdot \vec{v}_1 \vec{a}_1 \cdot \vec{v}_2 + \\ & \quad \hat{n} \times \vec{S}_1 \cdot \vec{v}_1 \vec{v}_1 \cdot \vec{a}_2 + \hat{n} \times \vec{S}_1 \cdot \vec{a}_1 \vec{v}_1 \cdot \vec{a}_2 + \frac{4}{3} \hat{n} \times \vec{S}_1 \cdot \vec{a}_1 \vec{v}_1 \cdot \vec{v}_2 + \frac{4}{3} \hat{n} \times \vec{S}_1 \cdot \vec{v}_1 \vec{v}_1 \cdot \vec{v}_2 \Big) m_1 m_2 G^2 + \frac{1}{r^2} \\ & \quad \left( -\frac{14}{3} \vec{S}_1 \times \vec{v}_1 \cdot \vec{v}_2 (\hat{n} \cdot \vec{v}_1)^2 - 2 \vec{S}_1 \times \vec{a}_1 \cdot \vec{v}_2 (\hat{n} \cdot \vec{v}_1)^2 - 2 \vec{S}_1 \times \vec{v}_1 \cdot \vec{a}_2 (\hat{n} \cdot \vec{v}_1)^2 + 8 \hat{n} \times \vec{S}_1 \cdot \vec{v}_1 \hat{n} \cdot \vec{a}_2 (\hat{n} \cdot \vec{v}_1)^2 + \right. \end{aligned}$$

$$\begin{aligned}
& \frac{56}{3} \hat{n} \times \vec{S}_1 \cdot \vec{v}_1 \hat{n} \cdot \vec{v}_2 (\hat{n} \cdot \vec{v}_1)^2 + 8 \hat{n} \times \vec{S}_1 \cdot \vec{a}_1 \hat{n} \cdot \vec{v}_2 (\hat{n} \cdot \vec{v}_1)^2 - 8 \hat{n} \times \vec{S}_1 \cdot \vec{v}_1 (\hat{n} \cdot \vec{v}_2)^2 \hat{n} \cdot \vec{v}_1 - \\
& 8 \hat{n} \times \vec{S}_1 \cdot \vec{a}_1 (\hat{n} \cdot \vec{v}_2)^2 \hat{n} \cdot \vec{v}_1 - 4 \vec{S}_1 \times \vec{v}_1 \cdot \vec{v}_2 \hat{n} \cdot \vec{a}_1 \hat{n} \cdot \vec{v}_1 + 4 \vec{S}_1 \times \vec{v}_1 \cdot \vec{v}_2 \hat{n} \cdot \vec{v}_2 \hat{n} \cdot \vec{v}_1 + 4 \vec{S}_1 \times \vec{a}_1 \cdot \vec{v}_2 \hat{n} \cdot \vec{v}_2 \hat{n} \cdot \vec{v}_1 + \\
& 16 \hat{n} \times \vec{S}_1 \cdot \vec{v}_1 \hat{n} \cdot \vec{a}_1 \hat{n} \cdot \vec{v}_2 \hat{n} \cdot \vec{v}_1 - 4 \hat{n} \times \vec{S}_1 \cdot \vec{v}_1 \vec{a}_1 \cdot \vec{v}_2 \hat{n} \cdot \vec{v}_1 - 4 \hat{n} \times \vec{S}_1 \cdot \vec{v}_1 \vec{v}_1 \cdot \vec{a}_2 \hat{n} \cdot \vec{v}_1 - \frac{28}{3} \hat{n} \times \vec{S}_1 \cdot \vec{v}_1 \vec{v}_1 \cdot \vec{v}_2 \hat{n} \cdot \vec{v}_1 - \\
& 4 \hat{n} \times \vec{S}_1 \cdot \vec{a}_1 \vec{v}_1 \cdot \vec{v}_2 \hat{n} \cdot \vec{v}_1 + 2 \hat{n} \times \vec{S}_1 \cdot \vec{v}_1 \vec{v}_2 \cdot \vec{v}_2 \hat{n} \cdot \vec{v}_1 + 2 \hat{n} \times \vec{S}_1 \cdot \vec{a}_1 \vec{v}_2 \cdot \vec{v}_2 \hat{n} \cdot \vec{v}_1 - 8 \hat{n} \times \vec{S}_1 \cdot \vec{v}_1 \hat{n} \cdot \vec{a}_1 (\hat{n} \cdot \vec{v}_2)^2 + \\
& 4 \vec{S}_1 \times \vec{v}_1 \cdot \vec{v}_2 \hat{n} \cdot \vec{a}_1 \hat{n} \cdot \vec{v}_2 - 2 \vec{S}_1 \times \vec{v}_1 \cdot \vec{v}_2 \vec{a}_1 \cdot \vec{v}_2 + 4 \hat{n} \times \vec{S}_1 \cdot \vec{v}_1 \hat{n} \cdot \vec{v}_2 \vec{a}_1 \cdot \vec{v}_2 + 2 \vec{S}_1 \times \vec{v}_1 \cdot \vec{v}_2 \vec{v}_1 \cdot \vec{a}_1 - \\
& 4 \hat{n} \times \vec{S}_1 \cdot \vec{v}_1 \hat{n} \cdot \vec{v}_2 \vec{v}_1 \cdot \vec{a}_1 + \frac{7}{3} \vec{S}_1 \times \vec{v}_1 \cdot \vec{v}_2 \vec{v}_1 \cdot \vec{v}_1 + \vec{S}_1 \times \vec{a}_1 \cdot \vec{v}_2 \vec{v}_1 \cdot \vec{v}_1 + \vec{S}_1 \times \vec{v}_1 \cdot \vec{a}_2 \vec{v}_1 \cdot \vec{v}_1 - 2 \hat{n} \times \vec{S}_1 \cdot \vec{v}_1 \hat{n} \cdot \vec{a}_2 \vec{v}_1 \cdot \vec{v}_1 - \\
& \frac{14}{3} \hat{n} \times \vec{S}_1 \cdot \vec{v}_1 \hat{n} \cdot \vec{v}_2 \vec{v}_1 \cdot \vec{v}_1 - 2 \hat{n} \times \vec{S}_1 \cdot \vec{a}_1 \hat{n} \cdot \vec{v}_2 \vec{v}_1 \cdot \vec{v}_1 - 2 \vec{S}_1 \times \vec{v}_1 \cdot \vec{v}_2 \vec{v}_1 \cdot \vec{v}_2 - 2 \vec{S}_1 \times \vec{a}_1 \cdot \vec{v}_2 \vec{v}_1 \cdot \vec{v}_2 - \\
& 4 \hat{n} \times \vec{S}_1 \cdot \vec{v}_1 \hat{n} \cdot \vec{a}_1 \vec{v}_1 \cdot \vec{v}_2 + 4 \hat{n} \times \vec{S}_1 \cdot \vec{v}_1 \hat{n} \cdot \vec{v}_2 \vec{v}_1 \cdot \vec{v}_2 + 4 \hat{n} \times \vec{S}_1 \cdot \vec{a}_1 \hat{n} \cdot \vec{v}_2 \vec{v}_1 \cdot \vec{v}_2 + 2 \hat{n} \times \vec{S}_1 \cdot \vec{v}_1 \hat{n} \cdot \vec{a}_1 \vec{v}_2 \cdot \vec{v}_2 \Big) m_1 m_2 G^2 + \\
& \frac{1}{r^3} \left( 8 \vec{S}_1 \times \vec{v}_1 \cdot \vec{v}_2 (\hat{n} \cdot \vec{v}_1)^3 - 48 \hat{n} \times \vec{S}_1 \cdot \vec{v}_1 \hat{n} \cdot \vec{v}_2 (\hat{n} \cdot \vec{v}_1)^3 + 48 \hat{n} \times \vec{S}_1 \cdot \vec{v}_1 (\hat{n} \cdot \vec{v}_2)^2 (\hat{n} \cdot \vec{v}_1)^2 - \right. \\
& 16 \vec{S}_1 \times \vec{v}_1 \cdot \vec{v}_2 \hat{n} \cdot \vec{v}_2 (\hat{n} \cdot \vec{v}_1)^2 + 24 \hat{n} \times \vec{S}_1 \cdot \vec{v}_1 \vec{v}_1 \cdot \vec{v}_2 (\hat{n} \cdot \vec{v}_1)^2 - 8 \hat{n} \times \vec{S}_1 \cdot \vec{v}_1 \vec{v}_2 \cdot \vec{v}_2 (\hat{n} \cdot \vec{v}_1)^2 - \\
& 6 \vec{S}_1 \times \vec{v}_1 \cdot \vec{v}_2 \vec{v}_1 \cdot \vec{v}_1 \hat{n} \cdot \vec{v}_1 + 24 \hat{n} \times \vec{S}_1 \cdot \vec{v}_1 \hat{n} \cdot \vec{v}_2 \vec{v}_1 \cdot \vec{v}_1 \hat{n} \cdot \vec{v}_1 + 8 \vec{S}_1 \times \vec{v}_1 \cdot \vec{v}_2 \vec{v}_1 \cdot \vec{v}_2 \hat{n} \cdot \vec{v}_1 - \\
& 32 \hat{n} \times \vec{S}_1 \cdot \vec{v}_1 \hat{n} \cdot \vec{v}_2 \vec{v}_1 \cdot \vec{v}_2 \hat{n} \cdot \vec{v}_1 + 4 \hat{n} \times \vec{S}_1 \cdot \vec{v}_1 (\vec{v}_1 \cdot \vec{v}_2)^2 - 8 \hat{n} \times \vec{S}_1 \cdot \vec{v}_1 (\hat{n} \cdot \vec{v}_2)^2 \vec{v}_1 \cdot \vec{v}_1 + \\
& \left. 4 \vec{S}_1 \times \vec{v}_1 \cdot \vec{v}_2 \hat{n} \cdot \vec{v}_2 \vec{v}_1 \cdot \vec{v}_1 - 6 \hat{n} \times \vec{S}_1 \cdot \vec{v}_1 \vec{v}_1 \cdot \vec{v}_1 \vec{v}_1 \cdot \vec{v}_2 + 2 \hat{n} \times \vec{S}_1 \cdot \vec{v}_1 \vec{v}_1 \cdot \vec{v}_1 \vec{v}_2 \cdot \vec{v}_2 \right) m_1 m_2 G^2 \Big\}
\end{aligned}$$

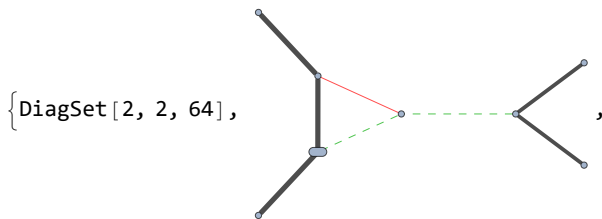

$$\begin{aligned}
& \frac{1}{r^2} G^2 m_1 m_2 \left( 8 \vec{v}_1 \cdot \vec{a}_1 \vec{S}_1 \times \vec{v}_1 \cdot \vec{v}_2 + 16 \vec{v}_1 \cdot \vec{v}_1 \vec{S}_1 \times \vec{a}_1 \cdot \vec{v}_2 - 8 \vec{v}_1 \cdot \vec{v}_2 \vec{S}_1 \times \vec{v}_1 \cdot \vec{a}_1 + \right. \\
& \left. 4 \vec{v}_2 \cdot \vec{v}_2 \vec{S}_1 \times \vec{a}_1 \cdot \vec{v}_2 + 16 \vec{v}_1 \cdot \vec{v}_1 \vec{S}_1 \times \vec{v}_1 \cdot \vec{v}_2 + 4 \vec{v}_2 \cdot \vec{v}_2 \vec{S}_1 \times \vec{v}_1 \cdot \vec{v}_2 \right) + \frac{1}{r^3} \\
& G^2 m_1 m_2 \left( -\frac{7}{4} (\vec{v}_1 \cdot \vec{v}_1)^2 \hat{n} \times \vec{S}_1 \cdot \vec{v}_2 - \frac{39}{4} \vec{v}_1 \cdot \vec{v}_1 \hat{n} \cdot \vec{v}_1 \vec{S}_1 \times \vec{v}_1 \cdot \vec{v}_2 - \frac{57}{4} \vec{v}_1 \cdot \vec{v}_2 \vec{v}_1 \cdot \vec{v}_1 \hat{n} \times \vec{S}_1 \cdot \vec{v}_1 - \right. \\
& \left. \frac{3}{2} \vec{v}_2 \cdot \vec{v}_2 \vec{v}_1 \cdot \vec{v}_1 \hat{n} \times \vec{S}_1 \cdot \vec{v}_2 - \frac{3}{4} (\vec{v}_2 \cdot \vec{v}_2)^2 \hat{n} \times \vec{S}_1 \cdot \vec{v}_2 - \frac{5}{2} \vec{v}_2 \cdot \vec{v}_2 \hat{n} \cdot \vec{v}_1 \vec{S}_1 \times \vec{v}_1 \cdot \vec{v}_2 - \frac{7}{2} \vec{v}_1 \cdot \vec{v}_2 \vec{v}_2 \cdot \vec{v}_2 \hat{n} \times \vec{S}_1 \cdot \vec{v}_1 \right) \Big\}
\end{aligned}$$

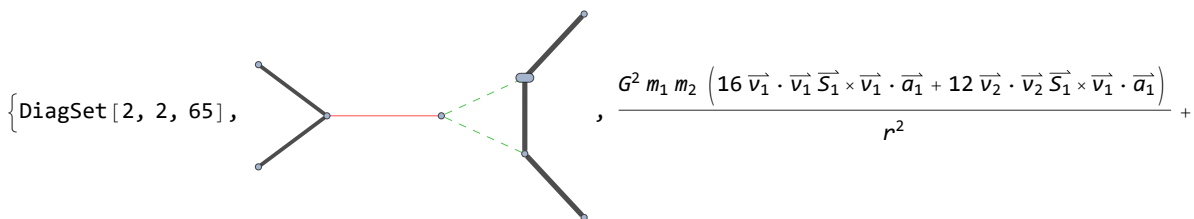

$$\frac{1}{r^3} G^2 m_1 m_2 \left( 8 (\vec{v}_1 \cdot \vec{v}_1)^2 \hat{n} \times \vec{S}_1 \cdot \vec{v}_1 + 12 \vec{v}_2 \cdot \vec{v}_2 \vec{v}_1 \cdot \vec{v}_1 \hat{n} \times \vec{S}_1 \cdot \vec{v}_1 + \frac{7}{4} (\vec{v}_2 \cdot \vec{v}_2)^2 \hat{n} \times \vec{S}_1 \cdot \vec{v}_1 \right) \Big\}$$

$\{\text{DiagSet}[2, 2, 66],$

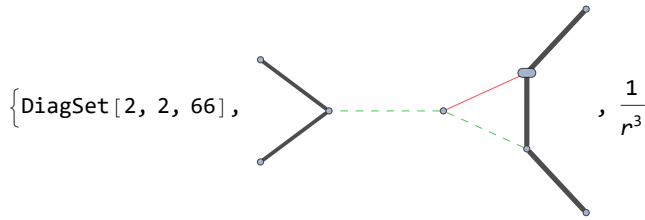

$, \frac{1}{r^3}$

$$\frac{G^2 m_1 m_2}{r^2} \left( 8 \vec{v}_1 \cdot \vec{v}_1 \hat{n} \cdot \vec{v}_1 \vec{S}_1 \times \vec{v}_1 \cdot \vec{v}_2 - 16 \vec{v}_1 \cdot \vec{v}_2 \vec{v}_1 \cdot \vec{v}_1 \hat{n} \times \vec{S}_1 \cdot \vec{v}_1 + 4 \vec{v}_2 \cdot \vec{v}_2 \hat{n} \cdot \vec{v}_1 \vec{S}_1 \times \vec{v}_1 \cdot \vec{v}_2 - 8 \vec{v}_1 \cdot \vec{v}_2 \vec{v}_2 \cdot \vec{v}_2 \hat{n} \times \vec{S}_1 \cdot \vec{v}_1 \right) -$$

$\{\text{DiagSet}[2, 2, 67],$

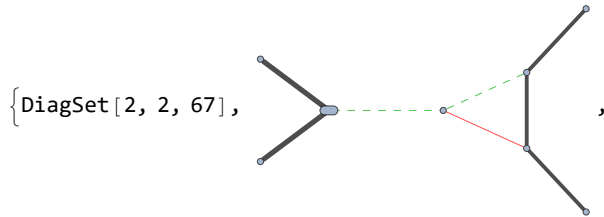

$,$

$$\frac{1}{r^2} G^2 m_2^2 \left( 8 \vec{a}_1 \cdot \vec{v}_1 \vec{S}_1 \times \vec{v}_1 \cdot \vec{v}_2 - 4 \vec{v}_1 \cdot \vec{v}_1 \vec{a}_1 \times \vec{S}_1 \cdot \vec{v}_2 - 8 \vec{v}_1 \cdot \vec{v}_2 \vec{a}_1 \times \vec{S}_1 \cdot \vec{v}_1 - \right.$$

$$\left. 16 \vec{v}_2 \cdot \vec{v}_2 \vec{a}_1 \times \vec{S}_1 \cdot \vec{v}_2 + 4 \vec{v}_1 \cdot \vec{v}_1 \vec{S}_1 \times \vec{v}_1 \cdot \vec{v}_2 + 16 \vec{v}_2 \cdot \vec{v}_2 \vec{S}_1 \times \vec{v}_1 \cdot \vec{v}_2 \right) + \frac{1}{r^3}$$

$$G^2 m_2^2 \left( -16 (\vec{v}_2 \cdot \vec{v}_2)^2 \hat{n} \times \vec{S}_1 \cdot \vec{v}_2 - 8 \vec{v}_2 \cdot \vec{v}_2 \hat{n} \cdot \vec{v}_1 \vec{S}_1 \times \vec{v}_1 \cdot \vec{v}_2 - 24 \vec{v}_1 \cdot \vec{v}_2 \vec{v}_2 \cdot \vec{v}_2 \hat{n} \times \vec{S}_1 \cdot \vec{v}_1 - \right.$$

$$\left. \vec{v}_1 \cdot \vec{v}_1 \hat{n} \cdot \vec{v}_1 \vec{S}_1 \times \vec{v}_1 \cdot \vec{v}_2 - 7 \vec{v}_1 \cdot \vec{v}_1 \vec{v}_1 \cdot \vec{v}_2 \hat{n} \times \vec{S}_1 \cdot \vec{v}_1 \right) \}$$

$\{\text{DiagSet}[2, 2, 68],$

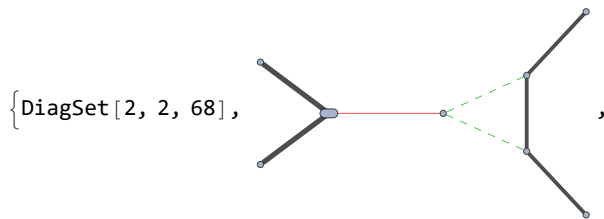

$,$

$$\frac{8 G^2 m_2^2 \vec{v}_2 \cdot \vec{v}_2 \vec{a}_1 \times \vec{S}_1 \cdot \vec{v}_1}{r^2} + \frac{G^2 m_2^2 \left( 16 (\vec{v}_2 \cdot \vec{v}_2)^2 \hat{n} \times \vec{S}_1 \cdot \vec{v}_1 + 8 \vec{v}_1 \cdot \vec{v}_1 \vec{v}_2 \cdot \vec{v}_2 \hat{n} \times \vec{S}_1 \cdot \vec{v}_1 \right)}{r^3} \}$$

$\{\text{DiagSet}[2, 2, 69],$

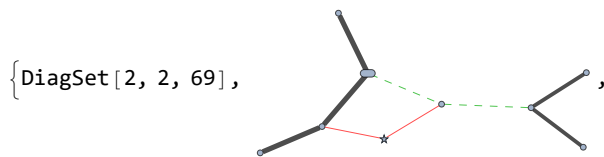

$,$

$$\frac{1}{r} \left( -4 \vec{S}_1 \times \vec{v}_1 \cdot \vec{a}_1 \hat{n} \cdot \vec{a}_2 - 8 \vec{S}_1 \times \vec{v}_1 \cdot \vec{a}_1 \hat{n} \cdot \vec{v}_2 - 4 \vec{S}_1 \times \vec{v}_1 \cdot \vec{a}_1 \hat{n} \cdot \vec{v}_2 + 6 \hat{n} \times \vec{S}_1 \cdot \vec{v}_2 \vec{v}_1 \cdot \vec{a}_1 + 6 \hat{n} \times \vec{S}_1 \cdot \vec{a}_2 \vec{v}_1 \cdot \vec{a}_1 - \right.$$

$$\left. 4 \hat{n} \times \vec{S}_1 \cdot \vec{v}_1 \vec{v}_1 \cdot \vec{a}_2 - 4 \hat{n} \times \vec{S}_1 \cdot \vec{a}_1 \vec{v}_1 \cdot \vec{a}_2 - 8 \hat{n} \times \vec{S}_1 \cdot \vec{a}_1 \vec{v}_1 \cdot \vec{v}_2 - 4 \hat{n} \times \vec{S}_1 \cdot \vec{v}_1 \vec{v}_1 \cdot \vec{v}_2 - 4 \hat{n} \times \vec{S}_1 \cdot \vec{a}_1 \vec{v}_1 \cdot \vec{v}_2 \right) m_1 m_2 G^2 +$$

$$\frac{1}{r^2} \left( \frac{1}{\vec{S}_1 \times \vec{v}_1 \cdot \vec{v}_2} (\hat{n} \cdot \vec{v}_1)^2 + \vec{S}_1 \times \vec{a}_1 \cdot \vec{v}_2 (\hat{n} \cdot \vec{v}_1)^2 - \vec{S}_1 \times \vec{v}_1 \cdot \vec{a}_2 (\hat{n} \cdot \vec{v}_1)^2 - \vec{S}_1 \times \vec{v}_1 \cdot \vec{v}_2 \hat{n} \cdot \vec{a}_1 \hat{n} \cdot \vec{v}_1 + \right.$$

$$\frac{11}{2} \vec{S}_1 \times \vec{v}_1 \cdot \vec{a}_1 \hat{n} \cdot \vec{v}_2 \hat{n} \cdot \vec{v}_1 + \hat{n} \times \vec{S}_1 \cdot \vec{v}_1 \vec{a}_1 \cdot \vec{v}_2 \hat{n} \cdot \vec{v}_1 - 18 \hat{n} \times \vec{S}_1 \cdot \vec{v}_2 \vec{v}_1 \cdot \vec{a}_1 \hat{n} \cdot \vec{v}_1 +$$

$$7 \hat{n} \times \vec{S}_1 \cdot \vec{v}_1 \vec{v}_1 \cdot \vec{a}_2 \hat{n} \cdot \vec{v}_1 + 3 \hat{n} \times \vec{S}_1 \cdot \vec{v}_2 \vec{v}_1 \cdot \vec{v}_1 \hat{n} \cdot \vec{v}_1 + 3 \hat{n} \times \vec{S}_1 \cdot \vec{a}_2 \vec{v}_1 \cdot \vec{v}_1 \hat{n} \cdot \vec{v}_1 + 11 \hat{n} \times \vec{S}_1 \cdot \vec{v}_1 \vec{v}_1 \cdot \vec{v}_2 \hat{n} \cdot \vec{v}_1 +$$

$$11 \hat{n} \times \vec{S}_1 \cdot \vec{a}_1 \vec{v}_1 \cdot \vec{v}_2 \hat{n} \cdot \vec{v}_1 + 2 \hat{n} \times \vec{S}_1 \cdot \vec{v}_2 \vec{v}_2 \cdot \vec{a}_2 \hat{n} \cdot \vec{v}_1 + \hat{n} \times \vec{S}_1 \cdot \vec{v}_2 \vec{v}_2 \cdot \vec{v}_2 \hat{n} \cdot \vec{v}_1 + \hat{n} \times \vec{S}_1 \cdot \vec{a}_2 \vec{v}_2 \cdot \vec{v}_2 \hat{n} \cdot \vec{v}_1 -$$

$$\begin{aligned}
& 8 \vec{S}_1 \times \vec{v}_1 \cdot \vec{a}_1 (\hat{n} \cdot \vec{v}_2)^2 - \frac{11}{2} \vec{S}_1 \times \vec{v}_1 \cdot \vec{v}_2 \vec{v}_1 \cdot \vec{a}_1 + \frac{9}{2} \hat{n} \times \vec{S}_1 \cdot \vec{v}_1 \hat{n} \cdot \vec{v}_2 \vec{v}_1 \cdot \vec{a}_1 + 12 \hat{n} \times \vec{S}_1 \cdot \vec{v}_2 \hat{n} \cdot \vec{v}_2 \vec{v}_1 \cdot \vec{a}_1 + \\
& 7 \frac{1}{2} \vec{S}_1 \times \vec{v}_1 \cdot \vec{v}_2 \vec{v}_1 \cdot \vec{v}_1 + \frac{11}{2} \vec{S}_1 \times \vec{a}_1 \cdot \vec{v}_2 \vec{v}_1 \cdot \vec{v}_1 + 5 \vec{S}_1 \times \vec{v}_1 \cdot \vec{a}_2 \vec{v}_1 \cdot \vec{v}_1 - 9 \hat{n} \times \vec{S}_1 \cdot \vec{v}_1 \hat{n} \cdot \vec{a}_2 \vec{v}_1 \cdot \vec{v}_1 - \\
& 9 \hat{n} \times \vec{S}_1 \cdot \vec{v}_1 \hat{n} \cdot \vec{v}_2 \vec{v}_1 \cdot \vec{v}_1 - \frac{9}{2} \hat{n} \times \vec{S}_1 \cdot \vec{a}_1 \hat{n} \cdot \vec{v}_2 \vec{v}_1 \cdot \vec{v}_1 + 4 \vec{S}_1 \times \vec{v}_1 \cdot \vec{v}_2 \vec{v}_1 \cdot \vec{v}_2 + 4 \vec{S}_1 \times \vec{a}_1 \cdot \vec{v}_2 \vec{v}_1 \cdot \vec{v}_2 - \\
& \frac{5}{2} \vec{S}_1 \times \vec{v}_1 \cdot \vec{a}_1 \vec{v}_1 \cdot \vec{v}_2 + 6 \hat{n} \times \vec{S}_1 \cdot \vec{v}_1 \hat{n} \cdot \vec{a}_1 \vec{v}_1 \cdot \vec{v}_2 - 8 \hat{n} \times \vec{S}_1 \cdot \vec{v}_1 \hat{n} \cdot \vec{v}_2 \vec{v}_1 \cdot \vec{v}_2 - 8 \hat{n} \times \vec{S}_1 \cdot \vec{a}_1 \hat{n} \cdot \vec{v}_2 \vec{v}_1 \cdot \vec{v}_2 + \\
& \vec{S}_1 \times \vec{v}_1 \cdot \vec{v}_2 \vec{v}_2 \cdot \vec{a}_2 - 3 \hat{n} \times \vec{S}_1 \cdot \vec{v}_1 \hat{n} \cdot \vec{v}_2 \vec{v}_2 \cdot \vec{a}_2 + \frac{1}{2} \vec{S}_1 \times \vec{v}_1 \cdot \vec{v}_2 \vec{v}_2 \cdot \vec{v}_2 + 4 \vec{S}_1 \times \vec{v}_1 \cdot \vec{a}_1 \vec{v}_2 \cdot \vec{v}_2 + \\
& \frac{1}{2} \vec{S}_1 \times \vec{v}_1 \cdot \vec{a}_2 \vec{v}_2 \cdot \vec{v}_2 - \frac{3}{2} \hat{n} \times \vec{S}_1 \cdot \vec{v}_1 \hat{n} \cdot \vec{a}_2 \vec{v}_2 \cdot \vec{v}_2 - \frac{3}{2} \hat{n} \times \vec{S}_1 \cdot \vec{v}_1 \hat{n} \cdot \vec{v}_2 \vec{v}_2 \cdot \vec{v}_2 \Big) m_1 m_2 G^2 + \frac{1}{r^3} \\
& \left( \vec{S}_1 \times \vec{v}_1 \cdot \vec{v}_2 (\hat{n} \cdot \vec{v}_1)^3 - 4 \vec{S}_1 \times \vec{v}_1 \cdot \vec{v}_2 \hat{n} \cdot \vec{v}_2 (\hat{n} \cdot \vec{v}_1)^2 - 9 \hat{n} \times \vec{S}_1 \cdot \vec{v}_2 \vec{v}_1 \cdot \vec{v}_1 (\hat{n} \cdot \vec{v}_1)^2 - 21 \hat{n} \times \vec{S}_1 \cdot \vec{v}_1 \vec{v}_1 \cdot \vec{v}_2 (\hat{n} \cdot \vec{v}_1)^2 - \right. \\
& 3 \hat{n} \times \vec{S}_1 \cdot \vec{v}_2 \vec{v}_2 \cdot \vec{v}_2 (\hat{n} \cdot \vec{v}_1)^2 - 12 \vec{S}_1 \times \vec{v}_1 \cdot \vec{v}_2 \vec{v}_1 \cdot \vec{v}_1 \hat{n} \cdot \vec{v}_1 + 24 \hat{n} \times \vec{S}_1 \cdot \vec{v}_1 \hat{n} \cdot \vec{v}_2 \vec{v}_1 \cdot \vec{v}_1 \hat{n} \cdot \vec{v}_1 + \\
& 12 \hat{n} \times \vec{S}_1 \cdot \vec{v}_2 \hat{n} \cdot \vec{v}_2 \vec{v}_1 \cdot \vec{v}_1 \hat{n} \cdot \vec{v}_1 - 5 \vec{S}_1 \times \vec{v}_1 \cdot \vec{v}_2 \vec{v}_1 \cdot \vec{v}_2 \hat{n} \cdot \vec{v}_1 + 28 \hat{n} \times \vec{S}_1 \cdot \vec{v}_1 \hat{n} \cdot \vec{v}_2 \vec{v}_1 \cdot \vec{v}_2 \hat{n} \cdot \vec{v}_1 - \\
& 2 \vec{S}_1 \times \vec{v}_1 \cdot \vec{v}_2 \vec{v}_2 \cdot \vec{v}_2 \hat{n} \cdot \vec{v}_1 + 4 \hat{n} \times \vec{S}_1 \cdot \vec{v}_1 \hat{n} \cdot \vec{v}_2 \vec{v}_2 \cdot \vec{v}_2 \hat{n} \cdot \vec{v}_1 + 4 \hat{n} \times \vec{S}_1 \cdot \vec{v}_2 \hat{n} \cdot \vec{v}_2 \vec{v}_2 \cdot \vec{v}_2 \hat{n} \cdot \vec{v}_1 - \\
& 7 \hat{n} \times \vec{S}_1 \cdot \vec{v}_1 (\vec{v}_1 \cdot \vec{v}_2)^2 + \frac{3}{2} \hat{n} \times \vec{S}_1 \cdot \vec{v}_1 (\vec{v}_2 \cdot \vec{v}_2)^2 - 36 \hat{n} \times \vec{S}_1 \cdot \vec{v}_1 (\hat{n} \cdot \vec{v}_2)^2 \vec{v}_1 \cdot \vec{v}_1 + 19 \vec{S}_1 \times \vec{v}_1 \cdot \vec{v}_2 \hat{n} \cdot \vec{v}_2 \vec{v}_1 \cdot \vec{v}_1 - \\
& 3 \hat{n} \times \vec{S}_1 \cdot \vec{v}_1 \vec{v}_1 \cdot \vec{v}_1 \vec{v}_1 \cdot \vec{v}_2 - 3 \hat{n} \times \vec{S}_1 \cdot \vec{v}_2 \vec{v}_1 \cdot \vec{v}_1 \vec{v}_1 \cdot \vec{v}_2 - 6 \hat{n} \times \vec{S}_1 \cdot \vec{v}_1 (\hat{n} \cdot \vec{v}_2)^2 \vec{v}_2 \cdot \vec{v}_2 + \frac{5}{2} \vec{S}_1 \times \vec{v}_1 \cdot \vec{v}_2 \hat{n} \cdot \vec{v}_2 \vec{v}_2 \cdot \vec{v}_2 + \\
& \left. 9 \hat{n} \times \vec{S}_1 \cdot \vec{v}_1 \vec{v}_1 \cdot \vec{v}_1 \vec{v}_2 \cdot \vec{v}_2 - \frac{1}{2} \hat{n} \times \vec{S}_1 \cdot \vec{v}_1 \vec{v}_1 \cdot \vec{v}_2 \vec{v}_2 \cdot \vec{v}_2 - \hat{n} \times \vec{S}_1 \cdot \vec{v}_2 \vec{v}_1 \cdot \vec{v}_2 \vec{v}_2 \cdot \vec{v}_2 \right) m_1 m_2 G^2 \Big\}
\end{aligned}$$

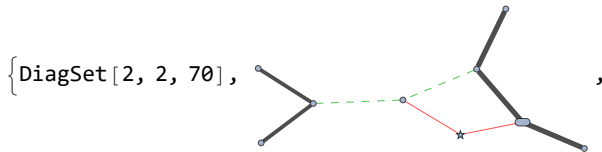

$$\begin{aligned}
& \frac{1}{r} \left( -8 \vec{S}_1 \times \vec{v}_1 \cdot \vec{v}_2 \hat{n} \cdot \vec{a}_1 - 8 \vec{S}_1 \times \vec{a}_1 \cdot \vec{v}_2 \hat{n} \cdot \vec{a}_1 - 8 \vec{S}_1 \times \vec{v}_1 \cdot \vec{a}_1 \hat{n} \cdot \vec{a}_2 - \right. \\
& \left. 8 \vec{S}_1 \times \vec{v}_1 \cdot \vec{a}_2 \hat{n} \cdot \vec{v}_1 - 8 \vec{S}_1 \times \vec{a}_1 \cdot \vec{a}_2 \hat{n} \cdot \vec{v}_1 + 8 \vec{S}_1 \times \vec{v}_1 \cdot \vec{a}_1 \hat{n} \cdot \vec{v}_2 \right) m_1 m_2 G^2 + \frac{1}{r^2} \\
& \left( 12 \vec{S}_1 \times \vec{v}_1 \cdot \vec{v}_2 (\hat{n} \cdot \vec{v}_1)^2 + 12 \vec{S}_1 \times \vec{a}_1 \cdot \vec{v}_2 (\hat{n} \cdot \vec{v}_1)^2 + 4 \vec{S}_1 \times \vec{v}_1 \cdot \vec{a}_2 (\hat{n} \cdot \vec{v}_1)^2 + 4 \vec{S}_1 \times \vec{v}_1 \cdot \vec{v}_2 \hat{n} \cdot \vec{a}_1 \hat{n} \cdot \vec{v}_1 - \right. \\
& 16 \vec{S}_1 \times \vec{v}_1 \cdot \vec{v}_2 \hat{n} \cdot \vec{v}_2 \hat{n} \cdot \vec{v}_1 - 16 \vec{S}_1 \times \vec{a}_1 \cdot \vec{v}_2 \hat{n} \cdot \vec{v}_2 \hat{n} \cdot \vec{v}_1 + 8 \vec{S}_1 \times \vec{v}_1 \cdot \vec{a}_1 \hat{n} \cdot \vec{v}_2 \hat{n} \cdot \vec{v}_1 - 4 \hat{n} \times \vec{S}_1 \cdot \vec{v}_1 \vec{a}_1 \cdot \vec{v}_2 \hat{n} \cdot \vec{v}_1 - \\
& 16 \vec{S}_1 \times \vec{v}_1 \cdot \vec{a}_1 (\hat{n} \cdot \vec{v}_2)^2 - 4 \hat{n} \times \vec{S}_1 \cdot \vec{v}_1 \hat{n} \cdot \vec{v}_2 \vec{v}_1 \cdot \vec{a}_1 - 8 \vec{S}_1 \times \vec{v}_1 \cdot \vec{v}_2 \vec{v}_1 \cdot \vec{v}_1 - 8 \vec{S}_1 \times \vec{a}_1 \cdot \vec{v}_2 \vec{v}_1 \cdot \vec{v}_1 - \\
& 4 \hat{n} \times \vec{S}_1 \cdot \vec{v}_1 \hat{n} \cdot \vec{a}_2 \vec{v}_1 \cdot \vec{v}_1 + 4 \hat{n} \times \vec{S}_1 \cdot \vec{v}_1 \hat{n} \cdot \vec{v}_2 \vec{v}_1 \cdot \vec{v}_1 + 4 \hat{n} \times \vec{S}_1 \cdot \vec{a}_1 \hat{n} \cdot \vec{v}_2 \vec{v}_1 \cdot \vec{v}_1 + 8 \vec{S}_1 \times \vec{v}_1 \cdot \vec{v}_2 \vec{v}_1 \cdot \vec{v}_2 + \\
& \left. 8 \vec{S}_1 \times \vec{a}_1 \cdot \vec{v}_2 \vec{v}_1 \cdot \vec{v}_2 - 12 \vec{S}_1 \times \vec{v}_1 \cdot \vec{a}_1 \vec{v}_1 \cdot \vec{v}_2 + 4 \hat{n} \times \vec{S}_1 \cdot \vec{v}_1 \hat{n} \cdot \vec{a}_1 \vec{v}_1 \cdot \vec{v}_2 + 8 \vec{S}_1 \times \vec{v}_1 \cdot \vec{a}_1 \vec{v}_2 \cdot \vec{v}_2 \right) m_1 m_2 G^2 + \\
& \frac{1}{r^3} \left( -8 \vec{S}_1 \times \vec{v}_1 \cdot \vec{v}_2 (\hat{n} \cdot \vec{v}_1)^3 + 16 \vec{S}_1 \times \vec{v}_1 \cdot \vec{v}_2 \hat{n} \cdot \vec{v}_2 (\hat{n} \cdot \vec{v}_1)^2 + 8 \vec{S}_1 \times \vec{v}_1 \cdot \vec{v}_2 \vec{v}_1 \cdot \vec{v}_1 \hat{n} \cdot \vec{v}_1 - \right. \\
& 8 \vec{S}_1 \times \vec{v}_1 \cdot \vec{v}_2 \vec{v}_1 \cdot \vec{v}_2 \hat{n} \cdot \vec{v}_1 - 16 \hat{n} \times \vec{S}_1 \cdot \vec{v}_1 (\hat{n} \cdot \vec{v}_2)^2 \vec{v}_1 \cdot \vec{v}_1 + 4 \vec{S}_1 \times \vec{v}_1 \cdot \vec{v}_2 \hat{n} \cdot \vec{v}_2 \vec{v}_1 \cdot \vec{v}_1 - \\
& \left. 4 \hat{n} \times \vec{S}_1 \cdot \vec{v}_1 \vec{v}_1 \cdot \vec{v}_1 \vec{v}_1 \cdot \vec{v}_2 + 4 \hat{n} \times \vec{S}_1 \cdot \vec{v}_1 \vec{v}_1 \cdot \vec{v}_1 \vec{v}_2 \cdot \vec{v}_2 \right) m_1 m_2 G^2 \Big\}
\end{aligned}$$

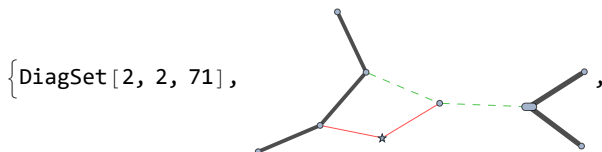



$$\begin{aligned}
& 3 \vec{S}_1 \times \vec{v}_1 \cdot \vec{v}_2 \vec{v}_2 \cdot \vec{a}_2 + \hat{n} \times \vec{S}_1 \cdot \vec{v}_1 \hat{n} \cdot \vec{v}_2 \vec{v}_2 \cdot \vec{a}_2 + \frac{3}{2} \vec{S}_1 \times \vec{v}_1 \cdot \vec{v}_2 \vec{v}_2 \cdot \vec{v}_2 - 4 \vec{S}_1 \times \vec{v}_1 \cdot \vec{a}_1 \vec{v}_2 \cdot \vec{v}_2 + \frac{3}{2} \vec{S}_1 \times \vec{v}_1 \cdot \vec{a}_2 \vec{v}_2 \cdot \vec{v}_2 + \\
& \frac{1}{2} \hat{n} \times \vec{S}_1 \cdot \vec{v}_1 \hat{n} \cdot \vec{a}_2 \vec{v}_2 \cdot \vec{v}_2 - \frac{1}{2} \hat{n} \times \vec{S}_1 \cdot \vec{v}_1 \hat{n} \cdot \vec{v}_2 \vec{v}_2 \cdot \vec{v}_2 - 6 \hat{n} \times \vec{S}_1 \cdot \vec{v}_2 \hat{n} \cdot \vec{v}_2 \vec{v}_2 \cdot \vec{v}_2 \Big) m_1 m_2 G^2 + \frac{1}{r^3} \\
& \left( \vec{S}_1 \times \vec{v}_1 \cdot \vec{v}_2 (\hat{n} \cdot \vec{v}_1)^3 + 4 \vec{S}_1 \times \vec{v}_1 \cdot \vec{v}_2 \hat{n} \cdot \vec{v}_2 (\hat{n} \cdot \vec{v}_1)^2 - 9 \hat{n} \times \vec{S}_1 \cdot \vec{v}_2 \vec{v}_1 \cdot \vec{v}_1 (\hat{n} \cdot \vec{v}_1)^2 - 5 \hat{n} \times \vec{S}_1 \cdot \vec{v}_1 \vec{v}_1 \cdot \vec{v}_2 (\hat{n} \cdot \vec{v}_1)^2 - \right. \\
& 3 \hat{n} \times \vec{S}_1 \cdot \vec{v}_2 \vec{v}_2 \cdot \vec{v}_2 (\hat{n} \cdot \vec{v}_1)^2 - 7 \vec{S}_1 \times \vec{v}_1 \cdot \vec{v}_2 \vec{v}_1 \cdot \vec{v}_1 \hat{n} \cdot \vec{v}_1 + 36 \hat{n} \times \vec{S}_1 \cdot \vec{v}_2 \hat{n} \cdot \vec{v}_2 \vec{v}_1 \cdot \vec{v}_1 \hat{n} \cdot \vec{v}_1 - \\
& 7 \vec{S}_1 \times \vec{v}_1 \cdot \vec{v}_2 \vec{v}_1 \cdot \vec{v}_2 \hat{n} \cdot \vec{v}_1 + 20 \hat{n} \times \vec{S}_1 \cdot \vec{v}_1 \hat{n} \cdot \vec{v}_2 \vec{v}_1 \cdot \vec{v}_2 \hat{n} \cdot \vec{v}_1 - 2 \vec{S}_1 \times \vec{v}_1 \cdot \vec{v}_2 \vec{v}_2 \cdot \vec{v}_2 \hat{n} \cdot \vec{v}_1 + \\
& 12 \hat{n} \times \vec{S}_1 \cdot \vec{v}_2 \hat{n} \cdot \vec{v}_2 \vec{v}_2 \cdot \vec{v}_2 \hat{n} \cdot \vec{v}_1 + 3 \hat{n} \times \vec{S}_1 \cdot \vec{v}_2 (\vec{v}_1 \cdot \vec{v}_1)^2 - 5 \hat{n} \times \vec{S}_1 \cdot \vec{v}_1 (\vec{v}_1 \cdot \vec{v}_2)^2 - \frac{1}{2} \hat{n} \times \vec{S}_1 \cdot \vec{v}_1 (\vec{v}_2 \cdot \vec{v}_2)^2 + \\
& 12 \hat{n} \times \vec{S}_1 \cdot \vec{v}_1 (\hat{n} \cdot \vec{v}_2)^2 \vec{v}_1 \cdot \vec{v}_1 + 3 \vec{S}_1 \times \vec{v}_1 \cdot \vec{v}_2 \hat{n} \cdot \vec{v}_2 \vec{v}_1 \cdot \vec{v}_1 + 2 \hat{n} \times \vec{S}_1 \cdot \vec{v}_1 \vec{v}_1 \cdot \vec{v}_1 \vec{v}_1 \cdot \vec{v}_2 - \\
& 9 \hat{n} \times \vec{S}_1 \cdot \vec{v}_2 \vec{v}_1 \cdot \vec{v}_1 \vec{v}_1 \cdot \vec{v}_2 + 2 \hat{n} \times \vec{S}_1 \cdot \vec{v}_1 (\hat{n} \cdot \vec{v}_2)^2 \vec{v}_2 \cdot \vec{v}_2 + \frac{5}{2} \vec{S}_1 \times \vec{v}_1 \cdot \vec{v}_2 \hat{n} \cdot \vec{v}_2 \vec{v}_2 \cdot \vec{v}_2 - 3 \hat{n} \times \vec{S}_1 \cdot \vec{v}_1 \vec{v}_1 \cdot \vec{v}_1 \vec{v}_2 \cdot \vec{v}_2 + \\
& \left. \hat{n} \times \vec{S}_1 \cdot \vec{v}_2 \vec{v}_1 \cdot \vec{v}_1 \vec{v}_2 \cdot \vec{v}_2 + \frac{1}{2} \hat{n} \times \vec{S}_1 \cdot \vec{v}_1 \vec{v}_1 \cdot \vec{v}_2 \vec{v}_2 \cdot \vec{v}_2 - 3 \hat{n} \times \vec{S}_1 \cdot \vec{v}_2 \vec{v}_1 \cdot \vec{v}_2 \vec{v}_2 \cdot \vec{v}_2 \right) m_1 m_2 G^2 + \\
& m_1 m_2 \left( \frac{8 \vec{S}_1 \times \vec{a}_1 \cdot \vec{a}_2 + 4 \vec{S}_1 \times \vec{v}_1 \cdot \vec{a}_2 + 4 \vec{S}_1 \times \vec{a}_1 \cdot \vec{a}_2}{\epsilon_d} - 16 \vec{S}_1 \times \vec{a}_1 \cdot \vec{a}_2 \log \left( \frac{r}{R_\theta} \right) - \right. \\
& \left. 8 \vec{S}_1 \times \vec{v}_1 \cdot \vec{a}_2 \log \left( \frac{r}{R_\theta} \right) - 8 \vec{S}_1 \times \vec{a}_1 \cdot \vec{a}_2 \log \left( \frac{r}{R_\theta} \right) \right) G^2 \Big\}
\end{aligned}$$

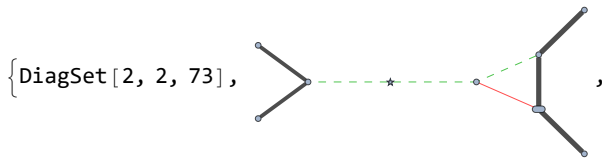

$$\begin{aligned}
& \frac{1}{r^2} G^2 m_1 m_2 \left( -8 (\hat{n} \cdot \vec{v}_1)^2 \vec{S}_1 \times \vec{v}_1 \cdot \vec{a}_2 + 8 \hat{n} \cdot \vec{v}_2 \hat{n} \cdot \vec{v}_1 \vec{S}_1 \times \vec{a}_1 \cdot \vec{v}_2 + 16 \vec{v}_1 \cdot \vec{a}_2 \hat{n} \cdot \vec{v}_1 \hat{n} \times \vec{S}_1 \cdot \vec{v}_1 + 8 \hat{n} \cdot \vec{a}_1 \hat{n} \cdot \vec{v}_2 \vec{S}_1 \times \vec{v}_1 \cdot \vec{v}_2 - \right. \\
& 16 \vec{a}_1 \cdot \vec{v}_2 \hat{n} \cdot \vec{v}_2 \hat{n} \times \vec{S}_1 \cdot \vec{v}_1 - 16 \vec{v}_1 \cdot \vec{v}_2 \hat{n} \cdot \vec{v}_2 \hat{n} \times \vec{S}_1 \cdot \vec{a}_1 + 4 \vec{a}_1 \cdot \vec{v}_2 \vec{S}_1 \times \vec{v}_1 \cdot \vec{v}_2 + 4 \vec{v}_1 \cdot \vec{v}_1 \vec{S}_1 \times \vec{v}_1 \cdot \vec{a}_2 + \\
& \left. 4 \vec{v}_1 \cdot \vec{v}_2 \vec{S}_1 \times \vec{a}_1 \cdot \vec{v}_2 + 8 \hat{n} \cdot \vec{v}_2 \hat{n} \cdot \vec{v}_1 \vec{S}_1 \times \vec{v}_1 \cdot \vec{v}_2 - 16 \vec{v}_1 \cdot \vec{v}_2 \hat{n} \cdot \vec{v}_2 \hat{n} \times \vec{S}_1 \cdot \vec{v}_1 + 4 \vec{v}_1 \cdot \vec{v}_2 \vec{S}_1 \times \vec{v}_1 \cdot \vec{v}_2 \right) + \\
& \frac{1}{r} G^2 m_1 m_2 \left( 4 \hat{n} \cdot \vec{a}_1 \vec{S}_1 \times \vec{v}_1 \cdot \vec{a}_2 + 4 \hat{n} \cdot \vec{v}_1 \vec{S}_1 \times \vec{v}_1 \cdot \vec{a}_2 + 4 \hat{n} \cdot \vec{v}_1 \vec{S}_1 \times \vec{a}_1 \cdot \vec{a}_2 - 8 \vec{a}_1 \cdot \vec{a}_2 \hat{n} \times \vec{S}_1 \cdot \vec{v}_1 - \right. \\
& 8 \vec{v}_1 \cdot \vec{a}_2 \hat{n} \times \vec{S}_1 \cdot \vec{v}_1 - 8 \vec{v}_1 \cdot \vec{a}_2 \hat{n} \times \vec{S}_1 \cdot \vec{a}_1 \Big) + \frac{1}{r^3} G^2 m_1 m_2 \left( -32 \hat{n} \cdot \vec{v}_2 (\hat{n} \cdot \vec{v}_1)^2 \vec{S}_1 \times \vec{v}_1 \cdot \vec{v}_2 + \right. \\
& \left. 64 \vec{v}_1 \cdot \vec{v}_2 \hat{n} \cdot \vec{v}_2 \hat{n} \cdot \vec{v}_1 \hat{n} \times \vec{S}_1 \cdot \vec{v}_1 - 16 (\vec{v}_1 \cdot \vec{v}_2)^2 \hat{n} \times \vec{S}_1 \cdot \vec{v}_1 + 8 \vec{v}_1 \cdot \vec{v}_1 \hat{n} \cdot \vec{v}_2 \vec{S}_1 \times \vec{v}_1 \cdot \vec{v}_2 \right) \Big\}
\end{aligned}$$

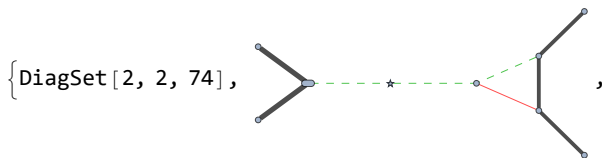

$$\begin{aligned}
& \frac{1}{r} G^2 \left( -2 \vec{a}_2 \times \vec{S}_1 \cdot \vec{v}_1 \hat{n} \cdot \vec{a}_1 - 10 \vec{a}_1 \times \vec{a}_2 \cdot \vec{S}_1 \hat{n} \cdot \vec{v}_1 - 10 \vec{a}_2 \times \vec{S}_1 \cdot \vec{v}_1 \hat{n} \cdot \vec{v}_1 - \right. \\
& 8 \vec{a}_1 \times \vec{S}_1 \cdot \vec{v}_2 \hat{n} \cdot \vec{v}_2 + 8 \vec{S}_1 \times \vec{v}_1 \cdot \vec{v}_2 \hat{n} \cdot \vec{v}_2 - 16 \vec{a}_1 \times \vec{S}_1 \cdot \vec{v}_2 \hat{n} \cdot \vec{v}_2 - 6 \hat{n} \times \vec{S}_1 \cdot \vec{v}_1 \vec{a}_1 \cdot \vec{a}_2 - \\
& 6 \hat{n} \times \vec{S}_1 \cdot \vec{v}_1 \vec{a}_2 \cdot \vec{v}_1 + 6 \hat{n} \times \vec{a}_1 \cdot \vec{S}_1 \vec{a}_2 \cdot \vec{v}_1 - 16 \hat{n} \times \vec{S}_1 \cdot \vec{v}_2 \vec{a}_2 \cdot \vec{v}_2 + 8 \hat{n} \times \vec{a}_2 \cdot \vec{S}_1 \vec{v}_2 \cdot \vec{v}_2 \Big) m_2^2 + \frac{1}{r^2} \\
& G^2 \left( 4 \vec{a}_2 \times \vec{S}_1 \cdot \vec{v}_1 (\hat{n} \cdot \vec{v}_1)^2 - 20 \vec{S}_1 \times \vec{v}_1 \cdot \vec{v}_2 \hat{n} \cdot \vec{v}_2 \hat{n} \cdot \vec{v}_1 + 20 \vec{a}_1 \times \vec{S}_1 \cdot \vec{v}_2 \hat{n} \cdot \vec{v}_2 \hat{n} \cdot \vec{v}_1 + 12 \hat{n} \times \vec{S}_1 \cdot \vec{v}_1 \vec{a}_2 \cdot \vec{v}_1 \hat{n} \cdot \vec{v}_1 + \right. \\
& \left. 32 \hat{n} \times \vec{S}_1 \cdot \vec{v}_2 \vec{a}_2 \cdot \vec{v}_2 \hat{n} \cdot \vec{v}_1 - 16 \hat{n} \times \vec{a}_2 \cdot \vec{S}_1 \vec{v}_2 \cdot \vec{v}_2 \hat{n} \cdot \vec{v}_1 - 4 \vec{S}_1 \times \vec{v}_1 \cdot \vec{v}_2 \hat{n} \cdot \vec{a}_1 \hat{n} \cdot \vec{v}_2 + 8 \vec{S}_1 \times \vec{v}_1 \cdot \vec{v}_2 \vec{a}_1 \cdot \vec{v}_2 - \right.
\end{aligned}$$

$$\begin{aligned}
 & 12 \hat{n} \times \vec{S}_1 \cdot \vec{v}_1 \hat{n} \cdot \vec{v}_2 \vec{a}_1 \cdot \vec{v}_2 + 16 \vec{S}_1 \times \vec{v}_1 \cdot \vec{v}_2 \vec{a}_2 \cdot \vec{v}_2 - 2 \vec{a}_2 \times \vec{S}_1 \cdot \vec{v}_1 \vec{v}_1 \cdot \vec{v}_1 + 16 \vec{S}_1 \times \vec{v}_1 \cdot \vec{v}_2 \vec{v}_1 \cdot \vec{v}_2 - 16 \vec{a}_1 \times \vec{S}_1 \cdot \vec{v}_2 \vec{v}_1 \cdot \vec{v}_2 - \\
 & 12 \hat{n} \times \vec{S}_1 \cdot \vec{v}_1 \hat{n} \cdot \vec{v}_2 \vec{v}_1 \cdot \vec{v}_2 + 12 \hat{n} \times \vec{a}_1 \cdot \vec{S}_1 \hat{n} \cdot \vec{v}_2 \vec{v}_1 \cdot \vec{v}_2 + 8 \vec{a}_2 \times \vec{S}_1 \cdot \vec{v}_1 \vec{v}_2 \cdot \vec{v}_2 - 16 \hat{n} \times \vec{S}_1 \cdot \vec{v}_2 \hat{n} \cdot \vec{v}_2 \vec{v}_2 \cdot \vec{v}_2 \Big) m_2^2 + \\
 & \frac{1}{r^3} G^2 \left( 16 \vec{S}_1 \times \vec{v}_1 \cdot \vec{v}_2 \hat{n} \cdot \vec{v}_2 (\hat{n} \cdot \vec{v}_1)^2 - 20 \vec{S}_1 \times \vec{v}_1 \cdot \vec{v}_2 \vec{v}_1 \cdot \vec{v}_2 \hat{n} \cdot \vec{v}_1 + 48 \hat{n} \times \vec{S}_1 \cdot \vec{v}_1 \hat{n} \cdot \vec{v}_2 \vec{v}_1 \cdot \vec{v}_2 \hat{n} \cdot \vec{v}_1 + \right. \\
 & 64 \hat{n} \times \vec{S}_1 \cdot \vec{v}_2 \hat{n} \cdot \vec{v}_2 \vec{v}_2 \cdot \vec{v}_2 \hat{n} \cdot \vec{v}_1 - 12 \hat{n} \times \vec{S}_1 \cdot \vec{v}_1 (\vec{v}_1 \cdot \vec{v}_2)^2 - 4 \vec{S}_1 \times \vec{v}_1 \cdot \vec{v}_2 \hat{n} \cdot \vec{v}_2 \vec{v}_1 \cdot \vec{v}_1 + \\
 & \left. 16 \vec{S}_1 \times \vec{v}_1 \cdot \vec{v}_2 \hat{n} \cdot \vec{v}_2 \vec{v}_2 \cdot \vec{v}_2 - 16 \hat{n} \times \vec{S}_1 \cdot \vec{v}_2 \vec{v}_1 \cdot \vec{v}_2 \vec{v}_2 \cdot \vec{v}_2 \right) m_2^2 + \\
 & G^2 \left( -8 \log \left( \frac{r}{R_\theta} \right) \frac{1}{\vec{a}_1 \times \vec{a}_2 \cdot \vec{S}_1} + 4 \frac{1}{\vec{a}_1 \times \vec{a}_2 \cdot \vec{S}_1} + 8 \vec{a}_1 \times \vec{a}_2 \cdot \vec{S}_1 + 4 \vec{a}_2 \times \vec{S}_1 \cdot \vec{v}_1 - 16 \vec{a}_1 \times \vec{a}_2 \cdot \vec{S}_1 \log \left( \frac{r}{R_\theta} \right) - \right. \\
 & \left. 8 \vec{a}_2 \times \vec{S}_1 \cdot \vec{v}_1 \log \left( \frac{r}{R_\theta} \right) + \frac{4 \frac{1}{\vec{a}_1 \times \vec{a}_2 \cdot \vec{S}_1} + 8 \vec{a}_1 \times \vec{a}_2 \cdot \vec{S}_1 + 4 \vec{a}_2 \times \vec{S}_1 \cdot \vec{v}_1}{\epsilon_d} \right) m_2^2 \Big\}
 \end{aligned}$$

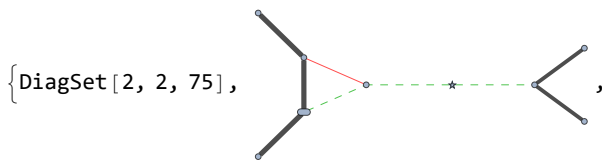

$$\begin{aligned}
 & \frac{1}{r} \left( -\frac{5}{2} \vec{S}_1 \times \vec{v}_1 \cdot \vec{a}_2 \hat{n} \cdot \vec{a}_1 - \frac{21}{2} \vec{S}_1 \times \vec{v}_1 \cdot \vec{a}_2 \hat{n} \cdot \vec{v}_1 - \frac{21}{2} \vec{S}_1 \times \vec{a}_1 \cdot \vec{a}_2 \hat{n} \cdot \vec{v}_1 + 16 \vec{S}_1 \times \vec{a}_1 \cdot \vec{v}_2 \hat{n} \cdot \vec{v}_2 + \right. \\
 & 8 \vec{S}_1 \times \vec{v}_1 \cdot \vec{v}_2 \hat{n} \cdot \vec{v}_2 + 8 \vec{S}_1 \times \vec{a}_1 \cdot \vec{v}_2 \hat{n} \cdot \vec{v}_2 - \frac{7}{2} \hat{n} \times \vec{S}_1 \cdot \vec{v}_1 \vec{a}_1 \cdot \vec{a}_2 - 3 \hat{n} \times \vec{S}_1 \cdot \vec{a}_2 \vec{v}_1 \cdot \vec{a}_1 - \frac{7}{2} \hat{n} \times \vec{S}_1 \cdot \vec{v}_1 \vec{v}_1 \cdot \vec{a}_2 - \\
 & \left. \frac{7}{2} \hat{n} \times \vec{S}_1 \cdot \vec{a}_1 \vec{v}_1 \cdot \vec{a}_2 - \frac{3}{2} \hat{n} \times \vec{S}_1 \cdot \vec{a}_2 \vec{v}_1 \cdot \vec{v}_1 - \hat{n} \times \vec{S}_1 \cdot \vec{v}_2 \vec{v}_2 \cdot \vec{a}_2 - \frac{1}{2} \hat{n} \times \vec{S}_1 \cdot \vec{a}_2 \vec{v}_2 \cdot \vec{v}_2 \right) m_1 m_2 G^2 + \frac{1}{r^2} \\
 & \left( 5 \vec{S}_1 \times \vec{v}_1 \cdot \vec{a}_2 (\hat{n} \cdot \vec{v}_1)^2 - 21 \vec{S}_1 \times \vec{v}_1 \cdot \vec{v}_2 \hat{n} \cdot \vec{v}_2 \hat{n} \cdot \vec{v}_1 - 21 \vec{S}_1 \times \vec{a}_1 \cdot \vec{v}_2 \hat{n} \cdot \vec{v}_2 \hat{n} \cdot \vec{v}_1 + 7 \hat{n} \times \vec{S}_1 \cdot \vec{v}_1 \vec{v}_1 \cdot \vec{a}_2 \hat{n} \cdot \vec{v}_1 + \right. \\
 & 3 \hat{n} \times \vec{S}_1 \cdot \vec{a}_2 \vec{v}_1 \cdot \vec{v}_1 \hat{n} \cdot \vec{v}_1 + 2 \hat{n} \times \vec{S}_1 \cdot \vec{v}_2 \vec{v}_2 \cdot \vec{a}_2 \hat{n} \cdot \vec{v}_1 + \hat{n} \times \vec{S}_1 \cdot \vec{a}_2 \vec{v}_2 \cdot \vec{v}_2 \hat{n} \cdot \vec{v}_1 - 5 \vec{S}_1 \times \vec{v}_1 \cdot \vec{v}_2 \hat{n} \cdot \vec{a}_1 \hat{n} \cdot \vec{v}_2 + \\
 & 6 \vec{S}_1 \times \vec{v}_1 \cdot \vec{v}_2 \vec{a}_1 \cdot \vec{v}_2 - 7 \hat{n} \times \vec{S}_1 \cdot \vec{v}_1 \hat{n} \cdot \vec{v}_2 \vec{a}_1 \cdot \vec{v}_2 - 6 \hat{n} \times \vec{S}_1 \cdot \vec{v}_2 \hat{n} \cdot \vec{v}_2 \vec{v}_1 \cdot \vec{a}_1 - \vec{S}_1 \times \vec{v}_1 \cdot \vec{a}_2 \vec{v}_1 \cdot \vec{v}_1 - \\
 & 3 \hat{n} \times \vec{S}_1 \cdot \vec{v}_2 \hat{n} \cdot \vec{v}_2 \vec{v}_1 \cdot \vec{v}_1 + 14 \vec{S}_1 \times \vec{v}_1 \cdot \vec{v}_2 \vec{v}_1 \cdot \vec{v}_2 + 14 \vec{S}_1 \times \vec{a}_1 \cdot \vec{v}_2 \vec{v}_1 \cdot \vec{v}_2 - 7 \hat{n} \times \vec{S}_1 \cdot \vec{v}_1 \hat{n} \cdot \vec{v}_2 \vec{v}_1 \cdot \vec{v}_2 - \\
 & \left. 7 \hat{n} \times \vec{S}_1 \cdot \vec{a}_1 \hat{n} \cdot \vec{v}_2 \vec{v}_1 \cdot \vec{v}_2 + \vec{S}_1 \times \vec{v}_1 \cdot \vec{v}_2 \vec{v}_2 \cdot \vec{a}_2 + \frac{1}{2} \vec{S}_1 \times \vec{v}_1 \cdot \vec{a}_2 \vec{v}_2 \cdot \vec{v}_2 - \hat{n} \times \vec{S}_1 \cdot \vec{v}_2 \hat{n} \cdot \vec{v}_2 \vec{v}_2 \cdot \vec{v}_2 \right) m_1 m_2 G^2 + \\
 & \frac{1}{r^3} \left( 20 \vec{S}_1 \times \vec{v}_1 \cdot \vec{v}_2 \hat{n} \cdot \vec{v}_2 (\hat{n} \cdot \vec{v}_1)^2 + 12 \hat{n} \times \vec{S}_1 \cdot \vec{v}_2 \hat{n} \cdot \vec{v}_2 \vec{v}_1 \cdot \vec{v}_1 \hat{n} \cdot \vec{v}_1 - 17 \vec{S}_1 \times \vec{v}_1 \cdot \vec{v}_2 \vec{v}_1 \cdot \vec{v}_2 \hat{n} \cdot \vec{v}_1 + \right. \\
 & 28 \hat{n} \times \vec{S}_1 \cdot \vec{v}_1 \hat{n} \cdot \vec{v}_2 \vec{v}_1 \cdot \vec{v}_2 \hat{n} \cdot \vec{v}_1 + 4 \hat{n} \times \vec{S}_1 \cdot \vec{v}_2 \hat{n} \cdot \vec{v}_2 \vec{v}_2 \cdot \vec{v}_2 \hat{n} \cdot \vec{v}_1 - 7 \hat{n} \times \vec{S}_1 \cdot \vec{v}_1 (\vec{v}_1 \cdot \vec{v}_2)^2 - \\
 & \left. 2 \vec{S}_1 \times \vec{v}_1 \cdot \vec{v}_2 \hat{n} \cdot \vec{v}_2 \vec{v}_1 \cdot \vec{v}_1 - 3 \hat{n} \times \vec{S}_1 \cdot \vec{v}_2 \vec{v}_1 \cdot \vec{v}_1 \vec{v}_1 \cdot \vec{v}_2 + \vec{S}_1 \times \vec{v}_1 \cdot \vec{v}_2 \hat{n} \cdot \vec{v}_2 \vec{v}_2 \cdot \vec{v}_2 - \hat{n} \times \vec{S}_1 \cdot \vec{v}_2 \vec{v}_1 \cdot \vec{v}_2 \vec{v}_2 \cdot \vec{v}_2 \right) m_1 m_2 G^2 + \\
 & m_1 m_2 \left( -16 \log \left( \frac{r}{R_\theta} \right) \frac{1}{\vec{S}_1 \times \vec{a}_1 \cdot \vec{a}_2} + 8 \frac{1}{\vec{S}_1 \times \vec{a}_1 \cdot \vec{a}_2} + 4 \vec{S}_1 \times \vec{v}_1 \cdot \vec{a}_2 + 4 \vec{S}_1 \times \vec{a}_1 \cdot \vec{a}_2 - 8 \vec{S}_1 \times \vec{v}_1 \cdot \vec{a}_2 \log \left( \frac{r}{R_\theta} \right) - \right. \\
 & \left. 8 \vec{S}_1 \times \vec{a}_1 \cdot \vec{a}_2 \log \left( \frac{r}{R_\theta} \right) + \frac{8 \frac{1}{\vec{S}_1 \times \vec{a}_1 \cdot \vec{a}_2} + 4 \vec{S}_1 \times \vec{v}_1 \cdot \vec{a}_2 + 4 \vec{S}_1 \times \vec{a}_1 \cdot \vec{a}_2}{\epsilon_d} \right) G^2 \Big\}
 \end{aligned}$$

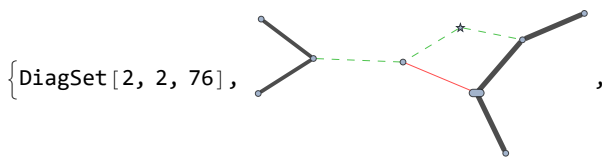

$$\{\text{DiagSet}[2, 2, 77],$$

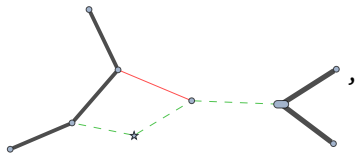

Printed by Wolfram Mathematica Student Edition



$$16 \vec{a}_1 \times \vec{a}_2 \cdot \vec{S}_1 \log\left(\frac{r}{R_0}\right) - 8 \vec{a}_2 \times \vec{S}_1 \cdot \vec{v}_1 \log\left(\frac{r}{R_0}\right) \Bigg\} m_2^2 \Bigg\}$$

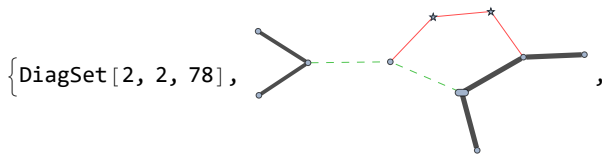

$$\begin{aligned} & \frac{1}{r} \left( \frac{7}{4} \hat{n} \times \vec{S}_1 \cdot \vec{v}_2 (\hat{n} \cdot \vec{a}_1)^2 + 2 \vec{S}_1 \times \vec{v}_1 \cdot \vec{v}_2 \hat{n} \cdot \vec{a}_1 + \vec{S}_1 \times \vec{a}_1 \cdot \vec{v}_2 \hat{n} \cdot \vec{a}_1 + 2 \vec{S}_1 \times \vec{v}_1 \cdot \vec{a}_2 \hat{n} \cdot \vec{a}_1 - \frac{2}{3} \vec{S}_1 \times \vec{v}_2 \cdot \vec{a}_2 \hat{n} \cdot \vec{a}_1 - \right. \\ & \quad \frac{1}{2} \hat{n} \times \vec{S}_1 \cdot \vec{v}_1 \hat{n} \cdot \vec{a}_2 \hat{n} \cdot \vec{a}_1 - \frac{4}{3} \hat{n} \times \vec{S}_1 \cdot \vec{v}_2 \hat{n} \cdot \vec{a}_2 \hat{n} \cdot \vec{a}_1 + \frac{7}{2} \hat{n} \times \vec{S}_1 \cdot \vec{v}_2 \hat{n} \cdot \vec{v}_1 \hat{n} \cdot \vec{a}_1 + \frac{7}{2} \hat{n} \times \vec{S}_1 \cdot \vec{a}_2 \hat{n} \cdot \vec{v}_1 \hat{n} \cdot \vec{a}_1 - \\ & \quad \frac{1}{2} \hat{n} \times \vec{S}_1 \cdot \vec{v}_1 \hat{n} \cdot \vec{v}_2 \hat{n} \cdot \vec{a}_1 - \frac{8}{3} \hat{n} \times \vec{S}_1 \cdot \vec{v}_2 \hat{n} \cdot \vec{v}_2 \hat{n} \cdot \vec{a}_1 - \frac{3}{2} \hat{n} \times \vec{S}_1 \cdot \vec{a}_1 \hat{n} \cdot \vec{v}_2 \hat{n} \cdot \vec{a}_1 - \frac{8}{3} \hat{n} \times \vec{S}_1 \cdot \vec{a}_2 \hat{n} \cdot \vec{v}_2 \hat{n} \cdot \vec{a}_1 - \\ & \quad \frac{5}{6} \hat{n} \times \vec{S}_1 \cdot \vec{a}_2 (\hat{n} \cdot \vec{v}_1)^2 - \frac{5}{12} \hat{n} \times \vec{S}_1 \cdot \vec{v}_2 (\hat{n} \cdot \vec{v}_1)^2 - \frac{5}{12} \hat{n} \times \vec{S}_1 \cdot \vec{a}_2 (\hat{n} \cdot \vec{v}_1)^2 + 2 \hat{n} \times \vec{S}_1 \cdot \vec{a}_1 (\hat{n} \cdot \vec{v}_2)^2 - \\ & \quad \frac{2}{3} \vec{S}_1 \times \vec{a}_1 \cdot \vec{v}_2 \hat{n} \cdot \vec{a}_2 - \vec{S}_1 \times \vec{v}_1 \cdot \vec{a}_1 \hat{n} \cdot \vec{a}_2 - \frac{4}{3} \vec{S}_1 \times \vec{v}_1 \cdot \vec{a}_2 \hat{n} \cdot \vec{v}_1 - \frac{2}{3} \vec{S}_1 \times \vec{v}_1 \cdot \vec{v}_2 \hat{n} \cdot \vec{v}_1 - \frac{2}{3} \vec{S}_1 \times \vec{v}_1 \cdot \vec{a}_2 \hat{n} \cdot \vec{v}_1 + \\ & \quad \frac{1}{2} \hat{n} \times \vec{S}_1 \cdot \vec{v}_1 \hat{n} \cdot \vec{a}_2 \hat{n} \cdot \vec{v}_1 + \hat{n} \times \vec{S}_1 \cdot \vec{v}_1 \hat{n} \cdot \vec{a}_2 \hat{n} \cdot \vec{v}_1 - \frac{5}{2} \hat{n} \times \vec{S}_1 \cdot \vec{a}_1 \hat{n} \cdot \vec{a}_2 \hat{n} \cdot \vec{v}_1 - \frac{1}{3} \vec{S}_1 \times \vec{a}_1 \cdot \vec{v}_2 \hat{n} \cdot \vec{v}_2 - \\ & \quad \vec{S}_1 \times \vec{v}_1 \cdot \vec{a}_1 \hat{n} \cdot \vec{v}_2 + \frac{1}{6} \vec{S}_1 \times \vec{a}_1 \cdot \vec{a}_2 \hat{n} \cdot \vec{v}_2 + 3 \hat{n} \times \vec{S}_1 \cdot \vec{a}_1 \hat{n} \cdot \vec{a}_2 \hat{n} \cdot \vec{v}_2 - \frac{5}{2} \hat{n} \times \vec{S}_1 \cdot \vec{a}_1 \hat{n} \cdot \vec{v}_1 \hat{n} \cdot \vec{v}_2 + \\ & \quad \frac{1}{2} \hat{n} \times \vec{S}_1 \cdot \vec{v}_1 \hat{n} \cdot \vec{v}_1 \hat{n} \cdot \vec{v}_2 + \frac{1}{4} \hat{n} \times \vec{S}_1 \cdot \vec{v}_2 \vec{a}_1 \cdot \vec{a}_1 - \frac{1}{2} \hat{n} \times \vec{S}_1 \cdot \vec{v}_1 \vec{a}_1 \cdot \vec{a}_2 + \frac{2}{3} \hat{n} \times \vec{S}_1 \cdot \vec{v}_2 \vec{a}_1 \cdot \vec{a}_2 - \frac{1}{2} \hat{n} \times \vec{S}_1 \cdot \vec{v}_1 \vec{a}_1 \cdot \vec{v}_2 + \\ & \quad \frac{4}{3} \hat{n} \times \vec{S}_1 \cdot \vec{v}_2 \vec{a}_1 \cdot \vec{v}_2 + \frac{4}{3} \hat{n} \times \vec{S}_1 \cdot \vec{a}_2 \vec{a}_1 \cdot \vec{v}_2 + \frac{1}{2} \hat{n} \times \vec{S}_1 \cdot \vec{v}_1 \vec{v}_1 \cdot \vec{a}_2 + \frac{1}{2} \hat{n} \times \vec{S}_1 \cdot \vec{v}_2 \vec{v}_1 \cdot \vec{a}_1 + \frac{1}{2} \hat{n} \times \vec{S}_1 \cdot \vec{a}_2 \vec{v}_1 \cdot \vec{a}_1 + \\ & \quad \hat{n} \times \vec{S}_1 \cdot \vec{v}_1 \vec{v}_1 \cdot \vec{a}_2 + \frac{1}{2} \hat{n} \times \vec{S}_1 \cdot \vec{a}_1 \vec{v}_1 \cdot \vec{a}_2 - \frac{11}{6} \hat{n} \times \vec{S}_1 \cdot \vec{a}_2 \vec{v}_1 \cdot \vec{v}_1 - \frac{11}{12} \hat{n} \times \vec{S}_1 \cdot \vec{v}_2 \vec{v}_1 \cdot \vec{v}_1 - \frac{11}{12} \hat{n} \times \vec{S}_1 \cdot \vec{a}_2 \vec{v}_1 \cdot \vec{v}_1 + \\ & \quad \left. \frac{1}{2} \hat{n} \times \vec{S}_1 \cdot \vec{a}_1 \vec{v}_1 \cdot \vec{v}_2 + \frac{1}{2} \hat{n} \times \vec{S}_1 \cdot \vec{v}_1 \vec{v}_1 \cdot \vec{v}_2 - \frac{3}{2} \hat{n} \times \vec{S}_1 \cdot \vec{a}_1 \vec{v}_2 \cdot \vec{a}_2 - \hat{n} \times \vec{S}_1 \cdot \vec{a}_1 \vec{v}_2 \cdot \vec{v}_2 \right) m_1 m_2 G^2 + \\ & \frac{1}{r^2} \left( \frac{8}{3} \hat{n} \times \vec{S}_1 \cdot \vec{v}_2 (\hat{n} \cdot \vec{v}_1)^3 + \frac{8}{3} \hat{n} \times \vec{S}_1 \cdot \vec{a}_2 (\hat{n} \cdot \vec{v}_1)^3 + 2 \vec{S}_1 \times \vec{v}_1 \cdot \vec{v}_2 (\hat{n} \cdot \vec{v}_1)^2 - \frac{1}{4} \vec{S}_1 \times \vec{a}_1 \cdot \vec{v}_2 (\hat{n} \cdot \vec{v}_1)^2 + \right. \\ & \quad 2 \vec{S}_1 \times \vec{v}_1 \cdot \vec{a}_2 (\hat{n} \cdot \vec{v}_1)^2 - \frac{5}{12} \vec{S}_1 \times \vec{v}_2 \cdot \vec{a}_2 (\hat{n} \cdot \vec{v}_1)^2 - 7 \hat{n} \times \vec{S}_1 \cdot \vec{v}_2 \hat{n} \cdot \vec{a}_1 (\hat{n} \cdot \vec{v}_1)^2 - 3 \hat{n} \times \vec{S}_1 \cdot \vec{v}_1 \hat{n} \cdot \vec{a}_2 (\hat{n} \cdot \vec{v}_1)^2 - \\ & \quad \frac{5}{3} \hat{n} \times \vec{S}_1 \cdot \vec{v}_2 \hat{n} \cdot \vec{a}_2 (\hat{n} \cdot \vec{v}_1)^2 - 3 \hat{n} \times \vec{S}_1 \cdot \vec{v}_1 \hat{n} \cdot \vec{v}_2 (\hat{n} \cdot \vec{v}_1)^2 - \frac{10}{3} \hat{n} \times \vec{S}_1 \cdot \vec{v}_2 \hat{n} \cdot \vec{v}_2 (\hat{n} \cdot \vec{v}_1)^2 + \\ & \quad 6 \hat{n} \times \vec{S}_1 \cdot \vec{a}_1 \hat{n} \cdot \vec{v}_2 (\hat{n} \cdot \vec{v}_1)^2 - \frac{10}{3} \hat{n} \times \vec{S}_1 \cdot \vec{a}_2 \hat{n} \cdot \vec{v}_2 (\hat{n} \cdot \vec{v}_1)^2 + 4 \hat{n} \times \vec{S}_1 \cdot \vec{v}_1 (\hat{n} \cdot \vec{v}_2)^2 \hat{n} \cdot \vec{v}_1 - \\ & \quad 10 \hat{n} \times \vec{S}_1 \cdot \vec{a}_1 (\hat{n} \cdot \vec{v}_2)^2 \hat{n} \cdot \vec{v}_1 - \frac{7}{2} \vec{S}_1 \times \vec{v}_1 \cdot \vec{v}_2 \hat{n} \cdot \vec{a}_1 \hat{n} \cdot \vec{v}_1 - \frac{7}{3} \vec{S}_1 \times \vec{v}_1 \cdot \vec{v}_2 \hat{n} \cdot \vec{a}_2 \hat{n} \cdot \vec{v}_1 - \frac{11}{3} \vec{S}_1 \times \vec{v}_1 \cdot \vec{v}_2 \hat{n} \cdot \vec{v}_2 \hat{n} \cdot \vec{v}_1 + \\ & \quad \frac{5}{2} \vec{S}_1 \times \vec{a}_1 \cdot \vec{v}_2 \hat{n} \cdot \vec{v}_2 \hat{n} \cdot \vec{v}_1 + 3 \vec{S}_1 \times \vec{v}_1 \cdot \vec{a}_1 \hat{n} \cdot \vec{v}_2 \hat{n} \cdot \vec{v}_1 - \frac{19}{6} \vec{S}_1 \times \vec{v}_1 \cdot \vec{a}_2 \hat{n} \cdot \vec{v}_2 \hat{n} \cdot \vec{v}_1 + 14 \hat{n} \times \vec{S}_1 \cdot \vec{v}_2 \hat{n} \cdot \vec{a}_1 \hat{n} \cdot \vec{v}_2 \hat{n} \cdot \vec{v}_1 + \\ & \quad 6 \hat{n} \times \vec{S}_1 \cdot \vec{v}_1 \hat{n} \cdot \vec{a}_2 \hat{n} \cdot \vec{v}_2 \hat{n} \cdot \vec{v}_1 + \frac{3}{2} \hat{n} \times \vec{S}_1 \cdot \vec{v}_1 \vec{a}_1 \cdot \vec{v}_2 \hat{n} \cdot \vec{v}_1 - \frac{7}{2} \hat{n} \times \vec{S}_1 \cdot \vec{v}_2 \vec{a}_1 \cdot \vec{v}_2 \hat{n} \cdot \vec{v}_1 - \hat{n} \times \vec{S}_1 \cdot \vec{v}_2 \vec{v}_1 \cdot \vec{a}_1 \hat{n} \cdot \vec{v}_1 + \\ & \quad \frac{5}{6} \hat{n} \times \vec{S}_1 \cdot \vec{v}_2 \vec{v}_1 \cdot \vec{a}_2 \hat{n} \cdot \vec{v}_1 + 4 \hat{n} \times \vec{S}_1 \cdot \vec{v}_2 \vec{v}_1 \cdot \vec{v}_1 \hat{n} \cdot \vec{v}_1 + 4 \hat{n} \times \vec{S}_1 \cdot \vec{a}_2 \vec{v}_1 \cdot \vec{v}_1 \hat{n} \cdot \vec{v}_1 + \frac{5}{3} \hat{n} \times \vec{S}_1 \cdot \vec{v}_2 \vec{v}_1 \cdot \vec{v}_2 \hat{n} \cdot \vec{v}_1 - \\ & \quad \frac{3}{2} \hat{n} \times \vec{S}_1 \cdot \vec{a}_1 \vec{v}_1 \cdot \vec{v}_2 \hat{n} \cdot \vec{v}_1 + \frac{5}{3} \hat{n} \times \vec{S}_1 \cdot \vec{a}_2 \vec{v}_1 \cdot \vec{v}_2 \hat{n} \cdot \vec{v}_1 - \frac{3}{2} \hat{n} \times \vec{S}_1 \cdot \vec{v}_1 \vec{v}_2 \cdot \vec{a}_2 \hat{n} \cdot \vec{v}_1 - \hat{n} \times \vec{S}_1 \cdot \vec{v}_1 \vec{v}_2 \cdot \vec{v}_2 \hat{n} \cdot \vec{v}_1 + \\ & \quad \left. \frac{5}{2} \hat{n} \times \vec{S}_1 \cdot \vec{a}_1 \vec{v}_2 \cdot \vec{v}_2 \hat{n} \cdot \vec{v}_1 + 4 \hat{n} \times \vec{S}_1 \cdot \vec{a}_1 (\hat{n} \cdot \vec{v}_2)^3 - \frac{4}{3} \vec{S}_1 \times \vec{a}_1 \cdot \vec{v}_2 (\hat{n} \cdot \vec{v}_2)^2 - 2 \vec{S}_1 \times \vec{v}_1 \cdot \vec{a}_1 (\hat{n} \cdot \vec{v}_2)^2 - \right. \end{aligned}$$

$$\begin{aligned}
& 2 \hat{n} \times \vec{S}_1 \cdot \vec{v}_1 \hat{n} \cdot \vec{a}_1 (\hat{n} \cdot \vec{v}_2)^2 - \frac{16}{3} \hat{n} \times \vec{S}_1 \cdot \vec{v}_2 \hat{n} \cdot \vec{a}_1 (\hat{n} \cdot \vec{v}_2)^2 + \frac{9}{2} \vec{S}_1 \times \vec{v}_1 \cdot \vec{v}_2 \hat{n} \cdot \vec{a}_1 \hat{n} \cdot \vec{v}_2 - \frac{3}{2} \vec{S}_1 \times \vec{v}_1 \cdot \vec{v}_2 \vec{a}_1 \cdot \vec{v}_2 - \\
& \frac{1}{2} \hat{n} \times \vec{S}_1 \cdot \vec{v}_1 \hat{n} \cdot \vec{v}_2 \vec{a}_1 \cdot \vec{v}_2 + \frac{8}{3} \hat{n} \times \vec{S}_1 \cdot \vec{v}_2 \hat{n} \cdot \vec{v}_2 \vec{a}_1 \cdot \vec{v}_2 - \frac{1}{2} \vec{S}_1 \times \vec{v}_1 \cdot \vec{v}_2 \vec{v}_1 \cdot \vec{a}_1 + \hat{n} \times \vec{S}_1 \cdot \vec{v}_2 \hat{n} \cdot \vec{v}_2 \vec{v}_1 \cdot \vec{a}_1 - \\
& \frac{1}{3} \vec{S}_1 \times \vec{v}_1 \cdot \vec{v}_2 \vec{v}_1 \cdot \vec{a}_2 + \frac{3}{2} \hat{n} \times \vec{S}_1 \cdot \vec{v}_1 \hat{n} \cdot \vec{v}_2 \vec{v}_1 \cdot \vec{a}_2 + 2 \vec{S}_1 \times \vec{v}_1 \cdot \vec{v}_2 \vec{v}_1 \cdot \vec{v}_1 + \frac{5}{4} \vec{S}_1 \times \vec{a}_1 \cdot \vec{v}_2 \vec{v}_1 \cdot \vec{v}_1 + 2 \vec{S}_1 \times \vec{v}_1 \cdot \vec{a}_2 \vec{v}_1 \cdot \vec{v}_1 - \\
& \frac{11}{12} \vec{S}_1 \times \vec{v}_2 \cdot \vec{a}_2 \vec{v}_1 \cdot \vec{v}_1 + 4 \hat{n} \times \vec{S}_1 \cdot \vec{v}_2 \hat{n} \cdot \vec{a}_1 \vec{v}_1 \cdot \vec{v}_1 - 3 \hat{n} \times \vec{S}_1 \cdot \vec{v}_1 \hat{n} \cdot \vec{a}_2 \vec{v}_1 \cdot \vec{v}_1 - \frac{11}{6} \hat{n} \times \vec{S}_1 \cdot \vec{v}_2 \hat{n} \cdot \vec{a}_2 \vec{v}_1 \cdot \vec{v}_1 - \\
& 3 \hat{n} \times \vec{S}_1 \cdot \vec{v}_1 \hat{n} \cdot \vec{v}_2 \vec{v}_1 \cdot \vec{v}_1 - \frac{11}{3} \hat{n} \times \vec{S}_1 \cdot \vec{v}_2 \hat{n} \cdot \vec{v}_2 \vec{v}_1 \cdot \vec{v}_1 - \frac{3}{2} \hat{n} \times \vec{S}_1 \cdot \vec{a}_1 \hat{n} \cdot \vec{v}_2 \vec{v}_1 \cdot \vec{v}_1 - \frac{11}{3} \hat{n} \times \vec{S}_1 \cdot \vec{a}_2 \hat{n} \cdot \vec{v}_2 \vec{v}_1 \cdot \vec{v}_1 + \\
& \frac{1}{3} \vec{S}_1 \times \vec{v}_1 \cdot \vec{v}_2 \vec{v}_1 \cdot \vec{v}_2 - \frac{1}{2} \vec{S}_1 \times \vec{a}_1 \cdot \vec{v}_2 \vec{v}_1 \cdot \vec{v}_2 + \frac{5}{6} \vec{S}_1 \times \vec{v}_1 \cdot \vec{a}_2 \vec{v}_1 \cdot \vec{v}_2 - \frac{3}{2} \hat{n} \times \vec{S}_1 \cdot \vec{v}_1 \hat{n} \cdot \vec{a}_1 \vec{v}_1 \cdot \vec{v}_2 - \\
& \frac{7}{2} \hat{n} \times \vec{S}_1 \cdot \vec{v}_2 \hat{n} \cdot \vec{a}_1 \vec{v}_1 \cdot \vec{v}_2 + \hat{n} \times \vec{S}_1 \cdot \vec{v}_1 \hat{n} \cdot \vec{v}_2 \vec{v}_1 \cdot \vec{v}_2 + \frac{7}{2} \hat{n} \times \vec{S}_1 \cdot \vec{a}_1 \hat{n} \cdot \vec{v}_2 \vec{v}_1 \cdot \vec{v}_2 + \frac{2}{3} \vec{S}_1 \times \vec{a}_1 \cdot \vec{v}_2 \vec{v}_2 \cdot \vec{v}_2 + \\
& \vec{S}_1 \times \vec{v}_1 \cdot \vec{a}_1 \vec{v}_2 \cdot \vec{v}_2 + \frac{1}{2} \hat{n} \times \vec{S}_1 \cdot \vec{v}_1 \hat{n} \cdot \vec{a}_1 \vec{v}_2 \cdot \vec{v}_2 + \frac{4}{3} \hat{n} \times \vec{S}_1 \cdot \vec{v}_2 \hat{n} \cdot \vec{a}_1 \vec{v}_2 \cdot \vec{v}_2 - 3 \hat{n} \times \vec{S}_1 \cdot \vec{a}_1 \hat{n} \cdot \vec{v}_2 \vec{v}_2 \cdot \vec{v}_2 \Big) m_1 m_2 G^2 + \frac{1}{r^3} \\
& \left( -\frac{55}{8} \hat{n} \times \vec{S}_1 \cdot \vec{v}_2 (\hat{n} \cdot \vec{v}_1)^4 - \frac{13}{3} \vec{S}_1 \times \vec{v}_1 \cdot \vec{v}_2 (\hat{n} \cdot \vec{v}_1)^3 + \frac{15}{2} \hat{n} \times \vec{S}_1 \cdot \vec{v}_1 \hat{n} \cdot \vec{v}_2 (\hat{n} \cdot \vec{v}_1)^3 + 16 \hat{n} \times \vec{S}_1 \cdot \vec{v}_2 \hat{n} \cdot \vec{v}_2 (\hat{n} \cdot \vec{v}_1)^3 - \right. \\
& 18 \hat{n} \times \vec{S}_1 \cdot \vec{v}_1 (\hat{n} \cdot \vec{v}_2)^2 (\hat{n} \cdot \vec{v}_1)^2 - 10 \hat{n} \times \vec{S}_1 \cdot \vec{v}_2 (\hat{n} \cdot \vec{v}_2)^2 (\hat{n} \cdot \vec{v}_1)^2 + 11 \vec{S}_1 \times \vec{v}_1 \cdot \vec{v}_2 \hat{n} \cdot \vec{v}_2 (\hat{n} \cdot \vec{v}_1)^2 - \\
& \frac{31}{4} \hat{n} \times \vec{S}_1 \cdot \vec{v}_2 \vec{v}_1 \cdot \vec{v}_1 (\hat{n} \cdot \vec{v}_1)^2 - \frac{3}{2} \hat{n} \times \vec{S}_1 \cdot \vec{v}_1 \vec{v}_1 \cdot \vec{v}_2 (\hat{n} \cdot \vec{v}_1)^2 - 8 \hat{n} \times \vec{S}_1 \cdot \vec{v}_2 \vec{v}_1 \cdot \vec{v}_2 (\hat{n} \cdot \vec{v}_1)^2 + \\
& 3 \hat{n} \times \vec{S}_1 \cdot \vec{v}_1 \vec{v}_2 \cdot \vec{v}_2 (\hat{n} \cdot \vec{v}_1)^2 + \frac{5}{3} \hat{n} \times \vec{S}_1 \cdot \vec{v}_2 \vec{v}_2 \cdot \vec{v}_2 (\hat{n} \cdot \vec{v}_1)^2 + 12 \hat{n} \times \vec{S}_1 \cdot \vec{v}_1 (\hat{n} \cdot \vec{v}_2)^3 \hat{n} \cdot \vec{v}_1 - \\
& \frac{28}{3} \vec{S}_1 \times \vec{v}_1 \cdot \vec{v}_2 (\hat{n} \cdot \vec{v}_2)^2 \hat{n} \cdot \vec{v}_1 - 5 \vec{S}_1 \times \vec{v}_1 \cdot \vec{v}_2 \vec{v}_1 \cdot \vec{v}_1 \hat{n} \cdot \vec{v}_1 + \frac{15}{2} \hat{n} \times \vec{S}_1 \cdot \vec{v}_1 \hat{n} \cdot \vec{v}_2 \vec{v}_1 \cdot \vec{v}_1 \hat{n} \cdot \vec{v}_1 + \\
& 16 \hat{n} \times \vec{S}_1 \cdot \vec{v}_2 \hat{n} \cdot \vec{v}_2 \vec{v}_1 \cdot \vec{v}_1 \hat{n} \cdot \vec{v}_1 - 4 \vec{S}_1 \times \vec{v}_1 \cdot \vec{v}_2 \vec{v}_1 \cdot \vec{v}_2 \hat{n} \cdot \vec{v}_1 + 6 \hat{n} \times \vec{S}_1 \cdot \vec{v}_1 \hat{n} \cdot \vec{v}_2 \vec{v}_1 \cdot \vec{v}_2 \hat{n} \cdot \vec{v}_1 + \\
& \frac{20}{3} \hat{n} \times \vec{S}_1 \cdot \vec{v}_2 \hat{n} \cdot \vec{v}_2 \vec{v}_1 \cdot \vec{v}_2 \hat{n} \cdot \vec{v}_1 + \frac{7}{3} \vec{S}_1 \times \vec{v}_1 \cdot \vec{v}_2 \vec{v}_2 \cdot \vec{v}_2 \hat{n} \cdot \vec{v}_1 - 6 \hat{n} \times \vec{S}_1 \cdot \vec{v}_1 \hat{n} \cdot \vec{v}_2 \vec{v}_2 \cdot \vec{v}_2 \hat{n} \cdot \vec{v}_1 + \\
& \frac{13}{8} \hat{n} \times \vec{S}_1 \cdot \vec{v}_2 (\vec{v}_1 \cdot \vec{v}_1)^2 - \frac{5}{6} \hat{n} \times \vec{S}_1 \cdot \vec{v}_2 (\vec{v}_1 \cdot \vec{v}_2)^2 - 12 \hat{n} \times \vec{S}_1 \cdot \vec{v}_1 (\hat{n} \cdot \vec{v}_2)^2 \vec{v}_1 \cdot \vec{v}_1 - \frac{22}{3} \hat{n} \times \vec{S}_1 \cdot \vec{v}_2 (\hat{n} \cdot \vec{v}_2)^2 \vec{v}_1 \cdot \vec{v}_1 + \\
& 7 \vec{S}_1 \times \vec{v}_1 \cdot \vec{v}_2 \hat{n} \cdot \vec{v}_2 \vec{v}_1 \cdot \vec{v}_1 + \frac{5}{3} \vec{S}_1 \times \vec{v}_1 \cdot \vec{v}_2 \hat{n} \cdot \vec{v}_2 \vec{v}_1 \cdot \vec{v}_2 - \frac{3}{2} \hat{n} \times \vec{S}_1 \cdot \vec{v}_1 \vec{v}_1 \cdot \vec{v}_1 \vec{v}_1 \cdot \vec{v}_2 - \\
& 4 \hat{n} \times \vec{S}_1 \cdot \vec{v}_2 \vec{v}_1 \cdot \vec{v}_1 \vec{v}_1 \cdot \vec{v}_2 + 3 \hat{n} \times \vec{S}_1 \cdot \vec{v}_1 \vec{v}_1 \cdot \vec{v}_1 \vec{v}_2 \cdot \vec{v}_2 + \frac{11}{6} \hat{n} \times \vec{S}_1 \cdot \vec{v}_2 \vec{v}_1 \cdot \vec{v}_1 \vec{v}_2 \cdot \vec{v}_2 \Big) m_1 m_2 G^2 + \\
& m_1 m_2 \left( -\frac{2}{3} \log\left(\frac{r}{R_\theta}\right) \vec{S}_1 \times \vec{a}_1 \cdot \vec{a}_2 + \frac{1}{9} \vec{S}_1 \times \vec{a}_1 \cdot \vec{a}_2 + \frac{1}{18} \vec{S}_1 \times \vec{a}_1 \cdot \vec{v}_2 + \frac{1}{18} \vec{S}_1 \times \vec{a}_1 \cdot \vec{a}_2 + \frac{1}{2} \hat{n} \times \vec{S}_1 \cdot \vec{a}_1 \hat{n} \cdot \vec{a}_2 - \right. \\
& \frac{4}{3} \hat{n} \times \vec{S}_1 \cdot \vec{a}_2 \hat{n} \cdot \vec{a}_1 - \frac{2}{3} \hat{n} \times \vec{S}_1 \cdot \vec{v}_2 \hat{n} \cdot \vec{a}_1 - \frac{2}{3} \hat{n} \times \vec{S}_1 \cdot \vec{a}_2 \hat{n} \cdot \vec{a}_1 + \hat{n} \times \vec{S}_1 \cdot \vec{a}_1 \hat{n} \cdot \vec{a}_2 + \frac{1}{2} \hat{n} \times \vec{S}_1 \cdot \vec{a}_1 \hat{n} \cdot \vec{v}_2 - \\
& \left. \frac{1}{3} \vec{S}_1 \times \vec{a}_1 \cdot \vec{v}_2 \log\left(\frac{r}{R_\theta}\right) - \frac{1}{3} \vec{S}_1 \times \vec{a}_1 \cdot \vec{a}_2 \log\left(\frac{r}{R_\theta}\right) + \frac{\frac{1}{3} \vec{S}_1 \times \vec{a}_1 \cdot \vec{a}_2 + \frac{1}{6} \vec{S}_1 \times \vec{a}_1 \cdot \vec{v}_2 + \frac{1}{6} \vec{S}_1 \times \vec{a}_1 \cdot \vec{a}_2}{\epsilon_d} \right) G^2 \Big\}
\end{aligned}$$

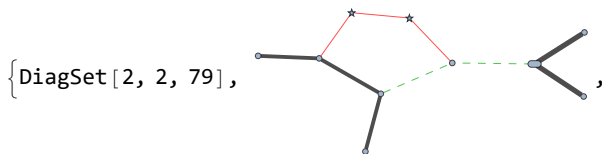

$$\begin{aligned}
& \frac{1}{r} G^2 \left( \frac{7}{3} \hat{n} \times \vec{S}_1 \cdot \vec{v}_2 (\hat{n} \cdot \vec{a}_2)^2 - \frac{4}{3} \vec{S}_1 \times \vec{v}_1 \cdot \vec{v}_2 \hat{n} \cdot \vec{a}_2 + \frac{2}{3} \vec{a}_1 \times \vec{S}_1 \cdot \vec{v}_2 \hat{n} \cdot \vec{a}_2 - 2 \vec{a}_2 \times \vec{S}_1 \cdot \vec{v}_1 \hat{n} \cdot \vec{a}_2 + \vec{a}_2 \times \vec{S}_1 \cdot \vec{v}_2 \hat{n} \cdot \vec{a}_2 - \right. \\
& \frac{4}{3} \hat{n} \times \vec{S}_1 \cdot \vec{v}_2 \hat{n} \cdot \vec{a}_1 \hat{n} \cdot \vec{a}_2 - \frac{8}{3} \hat{n} \times \vec{S}_1 \cdot \vec{v}_2 \hat{n} \cdot \vec{v}_1 \hat{n} \cdot \vec{a}_2 + 4 \hat{n} \times \vec{a}_2 \cdot \vec{S}_1 \hat{n} \cdot \vec{v}_1 \hat{n} \cdot \vec{a}_2 + \frac{8}{3} \hat{n} \times \vec{S}_1 \cdot \vec{v}_2 \hat{n} \cdot \vec{v}_2 \hat{n} \cdot \vec{a}_2 -
\end{aligned}$$

$$\begin{aligned}
& \frac{20}{3} \hat{n} \times \vec{a}_2 \cdot \vec{S}_1 \hat{n} \cdot \vec{v}_2 \hat{n} \cdot \vec{a}_2 + \frac{1}{3} \hat{n} \times \vec{a}_2 \cdot \vec{S}_1 (\hat{n} \cdot \vec{v}_2)^2 - \hat{n} \times \vec{S}_1 \cdot \vec{v}_2 (\hat{n} \cdot \vec{v}_2)^2 - \frac{4}{3} \hat{n} \times \vec{a}_2 \cdot \vec{S}_1 (\hat{n} \cdot \vec{v}_2)^2 + \\
& \frac{1}{3} \vec{a}_2 \times \vec{S}_1 \cdot \vec{v}_2 \hat{n} \cdot \vec{a}_1 + \frac{2}{3} \vec{a}_2 \times \vec{S}_1 \cdot \vec{v}_2 \hat{n} \cdot \vec{v}_1 - \frac{1}{3} \vec{a}_1 \times \vec{a}_2 \cdot \vec{S}_1 \hat{n} \cdot \vec{v}_2 - \frac{2}{3} \vec{a}_2 \times \vec{S}_1 \cdot \vec{v}_1 \hat{n} \cdot \vec{v}_2 - \frac{2}{3} \hat{n} \times \vec{S}_1 \cdot \vec{v}_2 \hat{n} \cdot \vec{a}_2 \hat{n} \cdot \vec{v}_2 + \\
& \frac{2}{3} \hat{n} \times \vec{a}_2 \cdot \vec{S}_1 \hat{n} \cdot \vec{a}_1 \hat{n} \cdot \vec{v}_2 + \frac{4}{3} \hat{n} \times \vec{a}_2 \cdot \vec{S}_1 \hat{n} \cdot \vec{v}_1 \hat{n} \cdot \vec{v}_2 + \frac{1}{3} \hat{n} \times \vec{S}_1 \cdot \vec{v}_2 \vec{a}_2 \cdot \vec{v}_2 + \frac{2}{3} \hat{n} \times \vec{S}_1 \cdot \vec{v}_2 \vec{a}_1 \cdot \vec{a}_2 - \\
& \frac{1}{3} \hat{n} \times \vec{a}_2 \cdot \vec{S}_1 \vec{a}_1 \cdot \vec{v}_2 + \frac{1}{3} \hat{n} \times \vec{S}_1 \cdot \vec{v}_2 \vec{a}_2 \cdot \vec{a}_2 + \frac{4}{3} \hat{n} \times \vec{S}_1 \cdot \vec{v}_2 \vec{a}_2 \cdot \vec{v}_1 - 2 \hat{n} \times \vec{a}_2 \cdot \vec{S}_1 \vec{a}_2 \cdot \vec{v}_1 + \frac{5}{3} \hat{n} \times \vec{S}_1 \cdot \vec{v}_2 \vec{a}_2 \cdot \vec{v}_2 + \\
& \frac{1}{3} \hat{n} \times \vec{a}_2 \cdot \vec{S}_1 \vec{a}_2 \cdot \vec{v}_2 - \frac{2}{3} \hat{n} \times \vec{a}_2 \cdot \vec{S}_1 \vec{v}_1 \cdot \vec{v}_2 + \frac{4}{3} \hat{n} \times \vec{a}_2 \cdot \vec{S}_1 \vec{v}_2 \cdot \vec{v}_2 - \hat{n} \times \vec{S}_1 \cdot \vec{v}_2 \vec{v}_2 \cdot \vec{v}_2 + \frac{11}{3} \hat{n} \times \vec{a}_2 \cdot \vec{S}_1 \vec{v}_2 \cdot \vec{v}_2 \Big) m_2^2 + \\
& \frac{1}{r^2} G^2 \left( -6 \hat{n} \times \vec{S}_1 \cdot \vec{v}_2 (\hat{n} \cdot \vec{v}_2)^3 - \frac{8}{3} \hat{n} \times \vec{a}_2 \cdot \vec{S}_1 (\hat{n} \cdot \vec{v}_2)^3 + 2 \vec{S}_1 \times \vec{v}_1 \cdot \vec{v}_2 (\hat{n} \cdot \vec{v}_2)^2 - \vec{a}_1 \times \vec{S}_1 \cdot \vec{v}_2 (\hat{n} \cdot \vec{v}_2)^2 - \right. \\
& \frac{4}{3} \vec{a}_2 \times \vec{S}_1 \cdot \vec{v}_1 (\hat{n} \cdot \vec{v}_2)^2 + \frac{7}{6} \vec{a}_2 \times \vec{S}_1 \cdot \vec{v}_2 (\hat{n} \cdot \vec{v}_2)^2 + 4 \hat{n} \times \vec{S}_1 \cdot \vec{v}_2 \hat{n} \cdot \vec{a}_1 (\hat{n} \cdot \vec{v}_2)^2 + \frac{10}{3} \hat{n} \times \vec{S}_1 \cdot \vec{v}_2 \hat{n} \cdot \vec{a}_2 (\hat{n} \cdot \vec{v}_2)^2 + \\
& 8 \hat{n} \times \vec{S}_1 \cdot \vec{v}_2 \hat{n} \cdot \vec{v}_1 (\hat{n} \cdot \vec{v}_2)^2 + \frac{16}{3} \hat{n} \times \vec{a}_2 \cdot \vec{S}_1 \hat{n} \cdot \vec{v}_1 (\hat{n} \cdot \vec{v}_2)^2 - \frac{8}{3} \hat{n} \times \vec{a}_2 \cdot \vec{S}_1 (\hat{n} \cdot \vec{v}_1)^2 \hat{n} \cdot \vec{v}_2 - \\
& \frac{8}{3} \vec{S}_1 \times \vec{v}_1 \cdot \vec{v}_2 \hat{n} \cdot \vec{a}_2 \hat{n} \cdot \vec{v}_2 + \frac{4}{3} \vec{a}_2 \times \vec{S}_1 \cdot \vec{v}_1 \hat{n} \cdot \vec{v}_1 \hat{n} \cdot \vec{v}_2 - \frac{32}{3} \hat{n} \times \vec{S}_1 \cdot \vec{v}_2 \hat{n} \cdot \vec{a}_2 \hat{n} \cdot \vec{v}_1 \hat{n} \cdot \vec{v}_2 - 2 \hat{n} \times \vec{S}_1 \cdot \vec{v}_2 \vec{a}_1 \cdot \vec{v}_2 \hat{n} \cdot \vec{v}_2 + \\
& \frac{8}{3} \hat{n} \times \vec{S}_1 \cdot \vec{v}_2 \vec{a}_2 \cdot \vec{v}_1 \hat{n} \cdot \vec{v}_2 + \frac{13}{3} \hat{n} \times \vec{S}_1 \cdot \vec{v}_2 \vec{a}_2 \cdot \vec{v}_2 \hat{n} \cdot \vec{v}_2 + \frac{2}{3} \hat{n} \times \vec{a}_2 \cdot \vec{S}_1 \vec{v}_1 \cdot \vec{v}_1 \hat{n} \cdot \vec{v}_2 - 4 \hat{n} \times \vec{S}_1 \cdot \vec{v}_2 \vec{v}_1 \cdot \vec{v}_2 \hat{n} \cdot \vec{v}_2 - \\
& \frac{8}{3} \hat{n} \times \vec{a}_2 \cdot \vec{S}_1 \vec{v}_1 \cdot \vec{v}_2 \hat{n} \cdot \vec{v}_2 - 6 \hat{n} \times \vec{S}_1 \cdot \vec{v}_2 \vec{v}_2 \cdot \vec{v}_2 \hat{n} \cdot \vec{v}_2 + 8 \hat{n} \times \vec{a}_2 \cdot \vec{S}_1 \vec{v}_2 \cdot \vec{v}_2 \hat{n} \cdot \vec{v}_2 - \frac{2}{3} \vec{a}_2 \times \vec{S}_1 \cdot \vec{v}_2 (\hat{n} \cdot \vec{v}_1)^2 + \\
& \frac{16}{3} \hat{n} \times \vec{S}_1 \cdot \vec{v}_2 \hat{n} \cdot \vec{a}_2 (\hat{n} \cdot \vec{v}_1)^2 + \frac{8}{3} \vec{S}_1 \times \vec{v}_1 \cdot \vec{v}_2 \hat{n} \cdot \vec{a}_2 \hat{n} \cdot \vec{v}_1 - \frac{4}{3} \vec{S}_1 \times \vec{v}_1 \cdot \vec{v}_2 \vec{a}_2 \cdot \vec{v}_1 - \frac{8}{3} \hat{n} \times \vec{S}_1 \cdot \vec{v}_2 \hat{n} \cdot \vec{v}_1 \vec{a}_2 \cdot \vec{v}_1 - \\
& \frac{5}{3} \vec{S}_1 \times \vec{v}_1 \cdot \vec{v}_2 \vec{a}_2 \cdot \vec{v}_2 - \frac{10}{3} \hat{n} \times \vec{S}_1 \cdot \vec{v}_2 \hat{n} \cdot \vec{v}_1 \vec{a}_2 \cdot \vec{v}_2 + \frac{1}{3} \vec{a}_2 \times \vec{S}_1 \cdot \vec{v}_2 \vec{v}_1 \cdot \vec{v}_1 - \frac{4}{3} \hat{n} \times \vec{S}_1 \cdot \vec{v}_2 \hat{n} \cdot \vec{a}_2 \vec{v}_1 \cdot \vec{v}_1 - \\
& \frac{2}{3} \vec{a}_2 \times \vec{S}_1 \cdot \vec{v}_1 \vec{v}_1 \cdot \vec{v}_2 + \frac{8}{3} \hat{n} \times \vec{S}_1 \cdot \vec{v}_2 \hat{n} \cdot \vec{a}_2 \vec{v}_1 \cdot \vec{v}_2 + \frac{4}{3} \hat{n} \times \vec{a}_2 \cdot \vec{S}_1 \hat{n} \cdot \vec{v}_1 \vec{v}_1 \cdot \vec{v}_2 + 2 \vec{S}_1 \times \vec{v}_1 \cdot \vec{v}_2 \vec{v}_2 \cdot \vec{v}_2 - \\
& \vec{a}_1 \times \vec{S}_1 \cdot \vec{v}_2 \vec{v}_2 \cdot \vec{v}_2 + \frac{11}{3} \vec{a}_2 \times \vec{S}_1 \cdot \vec{v}_1 \vec{v}_2 \cdot \vec{v}_2 + \frac{1}{6} \vec{a}_2 \times \vec{S}_1 \cdot \vec{v}_2 \vec{v}_2 \cdot \vec{v}_2 + 2 \hat{n} \times \vec{S}_1 \cdot \vec{v}_2 \hat{n} \cdot \vec{a}_1 \vec{v}_2 \cdot \vec{v}_2 - \\
& \frac{25}{3} \hat{n} \times \vec{S}_1 \cdot \vec{v}_2 \hat{n} \cdot \vec{a}_2 \vec{v}_2 \cdot \vec{v}_2 + 4 \hat{n} \times \vec{S}_1 \cdot \vec{v}_2 \hat{n} \cdot \vec{v}_1 \vec{v}_2 \cdot \vec{v}_2 - \frac{22}{3} \hat{n} \times \vec{a}_2 \cdot \vec{S}_1 \hat{n} \cdot \vec{v}_1 \vec{v}_2 \cdot \vec{v}_2 \Big) m_2^2 + \frac{1}{r^3} \\
& G^2 \left( -15 \hat{n} \times \vec{S}_1 \cdot \vec{v}_2 (\hat{n} \cdot \vec{v}_2)^4 + 6 \vec{S}_1 \times \vec{v}_1 \cdot \vec{v}_2 (\hat{n} \cdot \vec{v}_2)^3 + 36 \hat{n} \times \vec{S}_1 \cdot \vec{v}_2 \hat{n} \cdot \vec{v}_1 (\hat{n} \cdot \vec{v}_2)^3 - 24 \hat{n} \times \vec{S}_1 \cdot \vec{v}_2 (\hat{n} \cdot \vec{v}_1)^2 (\hat{n} \cdot \vec{v}_2)^2 - \right. \\
& 8 \vec{S}_1 \times \vec{v}_1 \cdot \vec{v}_2 \hat{n} \cdot \vec{v}_1 (\hat{n} \cdot \vec{v}_2)^2 + 4 \hat{n} \times \vec{S}_1 \cdot \vec{v}_2 \vec{v}_1 \cdot \vec{v}_1 (\hat{n} \cdot \vec{v}_2)^2 - 18 \hat{n} \times \vec{S}_1 \cdot \vec{v}_2 \vec{v}_1 \cdot \vec{v}_2 (\hat{n} \cdot \vec{v}_2)^2 - \\
& 12 \hat{n} \times \vec{S}_1 \cdot \vec{v}_2 \vec{v}_2 \cdot \vec{v}_2 (\hat{n} \cdot \vec{v}_2)^2 + 4 \vec{S}_1 \times \vec{v}_1 \cdot \vec{v}_2 \vec{v}_1 \cdot \vec{v}_2 \hat{n} \cdot \vec{v}_2 + 16 \hat{n} \times \vec{S}_1 \cdot \vec{v}_2 \hat{n} \cdot \vec{v}_1 \vec{v}_1 \cdot \vec{v}_2 \hat{n} \cdot \vec{v}_2 + \\
& 6 \vec{S}_1 \times \vec{v}_1 \cdot \vec{v}_2 \vec{v}_2 \cdot \vec{v}_2 \hat{n} \cdot \vec{v}_2 + 24 \hat{n} \times \vec{S}_1 \cdot \vec{v}_2 \hat{n} \cdot \vec{v}_1 \vec{v}_2 \cdot \vec{v}_2 \hat{n} \cdot \vec{v}_2 - 2 \hat{n} \times \vec{S}_1 \cdot \vec{v}_2 (\vec{v}_1 \cdot \vec{v}_2)^2 + 3 \hat{n} \times \vec{S}_1 \cdot \vec{v}_2 (\vec{v}_2 \cdot \vec{v}_2)^2 - \\
& 8 \hat{n} \times \vec{S}_1 \cdot \vec{v}_2 (\hat{n} \cdot \vec{v}_1)^2 \vec{v}_2 \cdot \vec{v}_2 - 4 \vec{S}_1 \times \vec{v}_1 \cdot \vec{v}_2 \hat{n} \cdot \vec{v}_1 \vec{v}_2 \cdot \vec{v}_2 + 2 \hat{n} \times \vec{S}_1 \cdot \vec{v}_2 \vec{v}_1 \cdot \vec{v}_1 \vec{v}_2 \cdot \vec{v}_2 - 6 \hat{n} \times \vec{S}_1 \cdot \vec{v}_2 \vec{v}_1 \cdot \vec{v}_2 \vec{v}_2 \cdot \vec{v}_2 \Big) m_2^2 + \\
& G^2 \left( -\frac{1}{3} \log\left(\frac{r}{R_\theta}\right) \vec{a}_2 \times \vec{a}_2 \cdot \vec{S}_1 + \frac{2}{9} \vec{a}_2 \times \vec{a}_2 \cdot \vec{S}_1 - \frac{2}{9} \vec{a}_2 \times \vec{S}_1 \cdot \vec{v}_2 - \frac{1}{3} \hat{n} \times \vec{a}_2 \cdot \vec{S}_1 \hat{n} \cdot \vec{a}_2 - \frac{2}{3} \hat{n} \times \vec{a}_2 \cdot \vec{S}_1 \hat{n} \cdot \vec{a}_2 + \frac{2}{3} \hat{n} \times \vec{S}_1 \cdot \vec{v}_2 \right. \\
& \left. \hat{n} \cdot \vec{a}_2 - 2 \hat{n} \times \vec{a}_2 \cdot \vec{S}_1 \hat{n} \cdot \vec{a}_2 - \frac{1}{3} \hat{n} \times \vec{a}_2 \cdot \vec{S}_1 \hat{n} \cdot \vec{v}_2 + \frac{1}{3} \vec{a}_2 \times \vec{S}_1 \cdot \vec{v}_2 \log\left(\frac{r}{R_\theta}\right) + \frac{\frac{1}{6} \vec{a}_2 \times \vec{a}_2 \cdot \vec{S}_1 - \frac{1}{6} \vec{a}_2 \times \vec{S}_1 \cdot \vec{v}_2}{\epsilon_d} \right) m_2^2 \Big\}
\end{aligned}$$

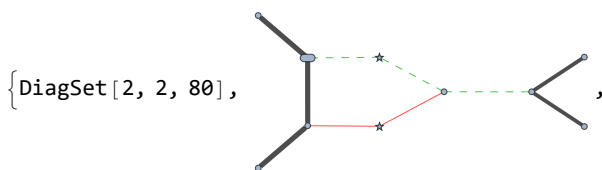

[illegible]

$$\begin{aligned}
 & \frac{1}{3} \hat{n} \times \vec{S}_1 \cdot \vec{v}_1 \hat{n} \cdot \vec{a}_2 \vec{v}_1 \cdot \vec{v}_1 - \hat{n} \times \vec{S}_1 \cdot \vec{v}_2 \hat{n} \cdot \vec{a}_2 \vec{v}_1 \cdot \vec{v}_1 - \frac{4}{3} \hat{n} \times \vec{S}_1 \cdot \vec{v}_1 \hat{n} \cdot \vec{v}_2 \vec{v}_1 \cdot \vec{v}_1 + \frac{5}{3} \hat{n} \times \vec{S}_1 \cdot \vec{v}_2 \hat{n} \cdot \vec{v}_2 \vec{v}_1 \cdot \vec{v}_1 + \\
 & \frac{1}{3} \hat{n} \times \vec{S}_1 \cdot \vec{a}_1 \hat{n} \cdot \vec{v}_2 \vec{v}_1 \cdot \vec{v}_1 - 2 \hat{n} \times \vec{S}_1 \cdot \vec{a}_2 \hat{n} \cdot \vec{v}_2 \vec{v}_1 \cdot \vec{v}_1 + \frac{11}{3} \vec{S}_1 \times \vec{v}_1 \cdot \vec{v}_2 \vec{v}_1 \cdot \vec{v}_2 + \frac{4}{3} \vec{S}_1 \times \vec{a}_1 \cdot \vec{v}_2 \vec{v}_1 \cdot \vec{v}_2 + \\
 & \frac{4}{3} \vec{S}_1 \times \vec{v}_1 \cdot \vec{a}_1 \vec{v}_1 \cdot \vec{v}_2 + 2 \vec{S}_1 \times \vec{v}_1 \cdot \vec{a}_2 \vec{v}_1 \cdot \vec{v}_2 - \hat{n} \times \vec{S}_1 \cdot \vec{v}_1 \hat{n} \cdot \vec{a}_1 \vec{v}_1 \cdot \vec{v}_2 + 3 \hat{n} \times \vec{S}_1 \cdot \vec{v}_2 \hat{n} \cdot \vec{a}_1 \vec{v}_1 \cdot \vec{v}_2 - \\
 & 2 \hat{n} \times \vec{S}_1 \cdot \vec{v}_1 \hat{n} \cdot \vec{a}_2 \vec{v}_1 \cdot \vec{v}_2 - 3 \hat{n} \times \vec{S}_1 \cdot \vec{v}_1 \hat{n} \cdot \vec{v}_2 \vec{v}_1 \cdot \vec{v}_2 - \frac{16}{3} \hat{n} \times \vec{S}_1 \cdot \vec{v}_2 \hat{n} \cdot \vec{v}_2 \vec{v}_1 \cdot \vec{v}_2 - \frac{5}{3} \hat{n} \times \vec{S}_1 \cdot \vec{a}_1 \hat{n} \cdot \vec{v}_2 \vec{v}_1 \cdot \vec{v}_2 - \\
 & \frac{4}{3} \vec{S}_1 \times \vec{v}_1 \cdot \vec{v}_2 \vec{v}_2 \cdot \vec{v}_2 - \frac{1}{3} \hat{n} \times \vec{S}_1 \cdot \vec{v}_1 \hat{n} \cdot \vec{a}_1 \vec{v}_2 \cdot \vec{v}_2 + 2 \hat{n} \times \vec{S}_1 \cdot \vec{v}_1 \hat{n} \cdot \vec{v}_2 \vec{v}_2 \cdot \vec{v}_2 \Big) m_1 m_2 G^2 + \frac{1}{r^3} \\
 & \left( -\frac{17}{4} \hat{n} \times \vec{S}_1 \cdot \vec{v}_2 (\hat{n} \cdot \vec{v}_1)^4 - 2 \vec{S}_1 \times \vec{v}_1 \cdot \vec{v}_2 (\hat{n} \cdot \vec{v}_1)^3 + \hat{n} \times \vec{S}_1 \cdot \vec{v}_1 \hat{n} \cdot \vec{v}_2 (\hat{n} \cdot \vec{v}_1)^3 + 36 \hat{n} \times \vec{S}_1 \cdot \vec{v}_2 \hat{n} \cdot \vec{v}_2 (\hat{n} \cdot \vec{v}_1)^3 - \right. \\
 & 8 \hat{n} \times \vec{S}_1 \cdot \vec{v}_1 (\hat{n} \cdot \vec{v}_2)^2 (\hat{n} \cdot \vec{v}_1)^2 - 36 \hat{n} \times \vec{S}_1 \cdot \vec{v}_2 (\hat{n} \cdot \vec{v}_2)^2 (\hat{n} \cdot \vec{v}_1)^2 + \frac{38}{3} \vec{S}_1 \times \vec{v}_1 \cdot \vec{v}_2 \hat{n} \cdot \vec{v}_2 (\hat{n} \cdot \vec{v}_1)^2 + \\
 & \frac{15}{2} \hat{n} \times \vec{S}_1 \cdot \vec{v}_2 \vec{v}_1 \cdot \vec{v}_1 (\hat{n} \cdot \vec{v}_1)^2 - \hat{n} \times \vec{S}_1 \cdot \vec{v}_1 \vec{v}_1 \cdot \vec{v}_2 (\hat{n} \cdot \vec{v}_1)^2 - 18 \hat{n} \times \vec{S}_1 \cdot \vec{v}_2 \vec{v}_1 \cdot \vec{v}_2 (\hat{n} \cdot \vec{v}_1)^2 + \\
 & \frac{4}{3} \hat{n} \times \vec{S}_1 \cdot \vec{v}_1 \vec{v}_2 \cdot \vec{v}_2 (\hat{n} \cdot \vec{v}_1)^2 + 6 \hat{n} \times \vec{S}_1 \cdot \vec{v}_2 \vec{v}_2 \cdot \vec{v}_2 (\hat{n} \cdot \vec{v}_1)^2 + 8 \hat{n} \times \vec{S}_1 \cdot \vec{v}_1 (\hat{n} \cdot \vec{v}_2)^3 \hat{n} \cdot \vec{v}_1 - \\
 & 8 \vec{S}_1 \times \vec{v}_1 \cdot \vec{v}_2 (\hat{n} \cdot \vec{v}_2)^2 \hat{n} \cdot \vec{v}_1 + 2 \vec{S}_1 \times \vec{v}_1 \cdot \vec{v}_2 \vec{v}_1 \cdot \vec{v}_1 \hat{n} \cdot \vec{v}_1 + \hat{n} \times \vec{S}_1 \cdot \vec{v}_1 \hat{n} \cdot \vec{v}_2 \vec{v}_1 \cdot \vec{v}_1 \hat{n} \cdot \vec{v}_1 - \\
 & 8 \hat{n} \times \vec{S}_1 \cdot \vec{v}_2 \hat{n} \cdot \vec{v}_2 \vec{v}_1 \cdot \vec{v}_1 \hat{n} \cdot \vec{v}_1 - \frac{22}{3} \vec{S}_1 \times \vec{v}_1 \cdot \vec{v}_2 \vec{v}_1 \cdot \vec{v}_2 \hat{n} \cdot \vec{v}_1 + \frac{28}{3} \hat{n} \times \vec{S}_1 \cdot \vec{v}_1 \hat{n} \cdot \vec{v}_2 \vec{v}_1 \cdot \vec{v}_2 \hat{n} \cdot \vec{v}_1 + \\
 & 24 \hat{n} \times \vec{S}_1 \cdot \vec{v}_2 \hat{n} \cdot \vec{v}_2 \vec{v}_1 \cdot \vec{v}_2 \hat{n} \cdot \vec{v}_1 + 2 \vec{S}_1 \times \vec{v}_1 \cdot \vec{v}_2 \vec{v}_2 \cdot \vec{v}_2 \hat{n} \cdot \vec{v}_1 - 4 \hat{n} \times \vec{S}_1 \cdot \vec{v}_1 \hat{n} \cdot \vec{v}_2 \vec{v}_2 \cdot \vec{v}_2 \hat{n} \cdot \vec{v}_1 - \\
 & \frac{5}{4} \hat{n} \times \vec{S}_1 \cdot \vec{v}_2 (\vec{v}_1 \cdot \vec{v}_1)^2 - \frac{5}{3} \hat{n} \times \vec{S}_1 \cdot \vec{v}_1 (\vec{v}_1 \cdot \vec{v}_2)^2 - 3 \hat{n} \times \vec{S}_1 \cdot \vec{v}_2 (\vec{v}_1 \cdot \vec{v}_2)^2 + \frac{4}{3} \hat{n} \times \vec{S}_1 \cdot \vec{v}_1 (\hat{n} \cdot \vec{v}_2)^2 \vec{v}_1 \cdot \vec{v}_1 - \\
 & 4 \hat{n} \times \vec{S}_1 \cdot \vec{v}_2 (\hat{n} \cdot \vec{v}_2)^2 \vec{v}_1 \cdot \vec{v}_1 - \frac{2}{3} \vec{S}_1 \times \vec{v}_1 \cdot \vec{v}_2 \hat{n} \cdot \vec{v}_2 \vec{v}_1 \cdot \vec{v}_1 - 8 \hat{n} \times \vec{S}_1 \cdot \vec{v}_1 (\hat{n} \cdot \vec{v}_2)^2 \vec{v}_1 \cdot \vec{v}_2 + \\
 & 6 \vec{S}_1 \times \vec{v}_1 \cdot \vec{v}_2 \hat{n} \cdot \vec{v}_2 \vec{v}_1 \cdot \vec{v}_2 + \hat{n} \times \vec{S}_1 \cdot \vec{v}_1 \vec{v}_1 \cdot \vec{v}_1 \vec{v}_1 \cdot \vec{v}_2 + 2 \hat{n} \times \vec{S}_1 \cdot \vec{v}_2 \vec{v}_1 \cdot \vec{v}_1 \vec{v}_1 \cdot \vec{v}_2 - \\
 & \left. \frac{1}{3} \hat{n} \times \vec{S}_1 \cdot \vec{v}_1 \vec{v}_1 \cdot \vec{v}_1 \vec{v}_2 \cdot \vec{v}_2 + \hat{n} \times \vec{S}_1 \cdot \vec{v}_2 \vec{v}_1 \cdot \vec{v}_1 \vec{v}_2 \cdot \vec{v}_2 + 2 \hat{n} \times \vec{S}_1 \cdot \vec{v}_1 \vec{v}_1 \cdot \vec{v}_2 \vec{v}_2 \cdot \vec{v}_2 \right) m_1 m_2 G^2 + \\
 & m_1 m_2 \left( -\frac{2}{3} \log\left(\frac{r}{R_\theta}\right) \vec{S}_1 \times \vec{a}_1 \cdot \vec{a}_2 + \frac{1}{9} \vec{S}_1 \times \vec{a}_1 \cdot \vec{a}_2 + \frac{1}{9} \vec{S}_1 \times \vec{v}_1 \cdot \vec{a}_2 + \frac{1}{9} \vec{S}_1 \times \vec{a}_1 \cdot \vec{v}_2 + \frac{1}{9} \vec{S}_1 \times \vec{v}_1 \cdot \vec{a}_2 - \right. \\
 & \frac{1}{3} \hat{n} \times \vec{S}_1 \cdot \vec{v}_1 \hat{n} \cdot \vec{a}_2 + \frac{4}{3} \hat{n} \times \vec{S}_1 \cdot \vec{a}_2 \hat{n} \cdot \vec{a}_1 + \frac{4}{3} \hat{n} \times \vec{S}_1 \cdot \vec{v}_2 \hat{n} \cdot \vec{a}_1 - \frac{1}{3} \hat{n} \times \vec{S}_1 \cdot \vec{a}_1 \hat{n} \cdot \vec{a}_2 - \frac{1}{3} \hat{n} \times \vec{S}_1 \cdot \vec{v}_1 \hat{n} \cdot \vec{a}_2 + \\
 & \frac{4}{3} \hat{n} \times \vec{S}_1 \cdot \vec{a}_2 \hat{n} \cdot \vec{v}_1 + \frac{4}{3} \hat{n} \times \vec{S}_1 \cdot \vec{a}_2 \hat{n} \cdot \vec{v}_1 - \frac{1}{3} \hat{n} \times \vec{S}_1 \cdot \vec{a}_1 \hat{n} \cdot \vec{v}_2 - \frac{2}{3} \vec{S}_1 \times \vec{v}_1 \cdot \vec{a}_2 \log\left(\frac{r}{R_\theta}\right) - \frac{2}{3} \vec{S}_1 \times \vec{a}_1 \cdot \vec{v}_2 \log\left(\frac{r}{R_\theta}\right) - \\
 & \left. \frac{2}{3} \vec{S}_1 \times \vec{v}_1 \cdot \vec{a}_2 \log\left(\frac{r}{R_\theta}\right) + \frac{\frac{1}{3} \vec{S}_1 \times \vec{a}_1 \cdot \vec{a}_2 + \frac{1}{3} \vec{S}_1 \times \vec{v}_1 \cdot \vec{a}_2 + \frac{1}{3} \vec{S}_1 \times \vec{a}_1 \cdot \vec{v}_2 + \frac{1}{3} \vec{S}_1 \times \vec{v}_1 \cdot \vec{a}_2}{\epsilon_d} \right) G^2 \Big\}
 \end{aligned}$$

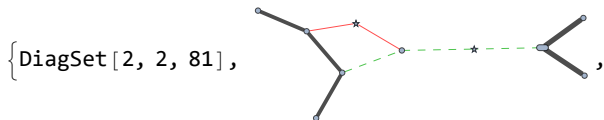

$$\begin{aligned}
 & \frac{1}{r} G^2 \left( -\frac{4}{3} \hat{n} \times \vec{S}_1 \cdot \vec{v}_2 (\hat{n} \cdot \vec{v}_2)^2 + \hat{n} \times \vec{a}_2 \cdot \vec{S}_1 (\hat{n} \cdot \vec{v}_2)^2 + \frac{2}{3} \vec{a}_1 \times \vec{a}_2 \cdot \vec{S}_1 \hat{n} \cdot \vec{v}_2 + \frac{4}{3} \vec{a}_2 \times \vec{S}_1 \cdot \vec{v}_1 \hat{n} \cdot \vec{v}_2 + \frac{2}{3} \vec{a}_2 \times \vec{S}_1 \cdot \vec{v}_2 \hat{n} \cdot \vec{v}_2 - \right. \\
 & \frac{4}{3} \hat{n} \times \vec{a}_2 \cdot \vec{S}_1 \hat{n} \cdot \vec{a}_1 \hat{n} \cdot \vec{v}_2 - \frac{10}{3} \hat{n} \times \vec{S}_1 \cdot \vec{v}_2 \hat{n} \cdot \vec{a}_2 \hat{n} \cdot \vec{v}_2 - \frac{8}{3} \hat{n} \times \vec{a}_2 \cdot \vec{S}_1 \hat{n} \cdot \vec{v}_1 \hat{n} \cdot \vec{v}_2 + \frac{2}{3} \vec{S}_1 \times \vec{v}_1 \cdot \vec{v}_2 \hat{n} \cdot \vec{a}_2 + \\
 & \frac{4}{3} \vec{S}_1 \times \vec{v}_1 \cdot \vec{v}_2 \hat{n} \cdot \vec{a}_2 - \frac{2}{3} \vec{a}_1 \times \vec{S}_1 \cdot \vec{v}_2 \hat{n} \cdot \vec{a}_2 + \frac{2}{3} \vec{a}_2 \times \vec{S}_1 \cdot \vec{v}_1 \hat{n} \cdot \vec{a}_2 + \frac{4}{3} \hat{n} \times \vec{S}_1 \cdot \vec{v}_2 \hat{n} \cdot \vec{a}_1 \hat{n} \cdot \vec{a}_2 - \\
 & \left. \frac{2}{3} \vec{a}_2 \times \vec{S}_1 \cdot \vec{v}_2 \hat{n} \cdot \vec{v}_1 + \frac{4}{3} \hat{n} \times \vec{S}_1 \cdot \vec{v}_2 \hat{n} \cdot \vec{a}_2 \hat{n} \cdot \vec{v}_1 + \frac{8}{3} \hat{n} \times \vec{S}_1 \cdot \vec{v}_2 \hat{n} \cdot \vec{a}_2 \hat{n} \cdot \vec{v}_1 - \frac{4}{3} \hat{n} \times \vec{a}_2 \cdot \vec{S}_1 \hat{n} \cdot \vec{a}_2 \hat{n} \cdot \vec{v}_1 - \right.
 \end{aligned}$$

$$\begin{aligned}
& \frac{2}{3} \hat{n} \times \vec{S}_1 \cdot \vec{v}_2 \vec{a}_2 \cdot \vec{v}_1 - \frac{2}{3} \hat{n} \times \vec{S}_1 \cdot \vec{v}_2 \vec{a}_1 \cdot \vec{a}_2 + \frac{2}{3} \hat{n} \times \vec{a}_2 \cdot \vec{S}_1 \vec{a}_1 \cdot \vec{v}_2 - \frac{4}{3} \hat{n} \times \vec{S}_1 \cdot \vec{v}_2 \vec{a}_2 \cdot \vec{v}_1 + \frac{2}{3} \hat{n} \times \vec{a}_2 \cdot \vec{S}_1 \vec{a}_2 \cdot \vec{v}_1 - \\
& \frac{4}{3} \hat{n} \times \vec{S}_1 \cdot \vec{v}_2 \vec{a}_2 \cdot \vec{v}_2 + \frac{4}{3} \hat{n} \times \vec{a}_2 \cdot \vec{S}_1 \vec{v}_1 \cdot \vec{v}_2 + \frac{2}{3} \hat{n} \times \vec{S}_1 \cdot \vec{v}_2 \vec{v}_2 \cdot \vec{v}_2 + \hat{n} \times \vec{a}_2 \cdot \vec{S}_1 \vec{v}_2 \cdot \vec{v}_2 \Big) m_2^2 + \frac{1}{r^2} \\
& G^2 \left( -4 \hat{n} \times \vec{S}_1 \cdot \vec{v}_2 (\hat{n} \cdot \vec{v}_2)^3 + \frac{8}{3} \vec{S}_1 \times \vec{v}_1 \cdot \vec{v}_2 (\hat{n} \cdot \vec{v}_2)^2 - \frac{4}{3} \vec{a}_1 \times \vec{S}_1 \cdot \vec{v}_2 (\hat{n} \cdot \vec{v}_2)^2 + \vec{a}_2 \times \vec{S}_1 \cdot \vec{v}_1 (\hat{n} \cdot \vec{v}_2)^2 + \right. \\
& \frac{16}{3} \hat{n} \times \vec{S}_1 \cdot \vec{v}_2 \hat{n} \cdot \vec{a}_1 (\hat{n} \cdot \vec{v}_2)^2 + \frac{32}{3} \hat{n} \times \vec{S}_1 \cdot \vec{v}_2 \hat{n} \cdot \vec{v}_1 (\hat{n} \cdot \vec{v}_2)^2 - 4 \hat{n} \times \vec{a}_2 \cdot \vec{S}_1 \hat{n} \cdot \vec{v}_1 (\hat{n} \cdot \vec{v}_2)^2 + \\
& \frac{16}{3} \hat{n} \times \vec{a}_2 \cdot \vec{S}_1 (\hat{n} \cdot \vec{v}_1)^2 \hat{n} \cdot \vec{v}_2 + \frac{10}{3} \vec{S}_1 \times \vec{v}_1 \cdot \vec{v}_2 \hat{n} \cdot \vec{a}_2 \hat{n} \cdot \vec{v}_2 - \frac{8}{3} \vec{a}_2 \times \vec{S}_1 \cdot \vec{v}_1 \hat{n} \cdot \vec{v}_1 \hat{n} \cdot \vec{v}_2 - \frac{4}{3} \vec{a}_2 \times \vec{S}_1 \cdot \vec{v}_2 \hat{n} \cdot \vec{v}_1 \hat{n} \cdot \vec{v}_2 + \\
& \frac{40}{3} \hat{n} \times \vec{S}_1 \cdot \vec{v}_2 \hat{n} \cdot \vec{a}_2 \hat{n} \cdot \vec{v}_1 \hat{n} \cdot \vec{v}_2 - \frac{8}{3} \hat{n} \times \vec{S}_1 \cdot \vec{v}_2 \vec{a}_1 \cdot \vec{v}_2 \hat{n} \cdot \vec{v}_2 - \frac{10}{3} \hat{n} \times \vec{S}_1 \cdot \vec{v}_2 \vec{a}_2 \cdot \vec{v}_1 \hat{n} \cdot \vec{v}_2 - \\
& \frac{4}{3} \hat{n} \times \vec{a}_2 \cdot \vec{S}_1 \vec{v}_1 \cdot \vec{v}_1 \hat{n} \cdot \vec{v}_2 - \frac{16}{3} \hat{n} \times \vec{S}_1 \cdot \vec{v}_2 \vec{v}_1 \cdot \vec{v}_2 \hat{n} \cdot \vec{v}_2 + 2 \hat{n} \times \vec{a}_2 \cdot \vec{S}_1 \vec{v}_1 \cdot \vec{v}_2 \hat{n} \cdot \vec{v}_2 - \frac{16}{3} \hat{n} \times \vec{S}_1 \cdot \vec{v}_2 \hat{n} \cdot \vec{a}_2 (\hat{n} \cdot \vec{v}_1)^2 - \\
& \frac{8}{3} \vec{S}_1 \times \vec{v}_1 \cdot \vec{v}_2 \hat{n} \cdot \vec{a}_2 \hat{n} \cdot \vec{v}_1 + \frac{4}{3} \vec{S}_1 \times \vec{v}_1 \cdot \vec{v}_2 \vec{a}_2 \cdot \vec{v}_1 + \frac{8}{3} \hat{n} \times \vec{S}_1 \cdot \vec{v}_2 \hat{n} \cdot \vec{v}_1 \vec{a}_2 \cdot \vec{v}_1 + \frac{4}{3} \vec{S}_1 \times \vec{v}_1 \cdot \vec{v}_2 \vec{a}_2 \cdot \vec{v}_2 + \\
& \frac{8}{3} \hat{n} \times \vec{S}_1 \cdot \vec{v}_2 \hat{n} \cdot \vec{v}_1 \vec{a}_2 \cdot \vec{v}_2 + \frac{4}{3} \hat{n} \times \vec{S}_1 \cdot \vec{v}_2 \hat{n} \cdot \vec{a}_2 \vec{v}_1 \cdot \vec{v}_1 + \frac{4}{3} \vec{a}_2 \times \vec{S}_1 \cdot \vec{v}_1 \vec{v}_1 \cdot \vec{v}_2 + \frac{2}{3} \vec{a}_2 \times \vec{S}_1 \cdot \vec{v}_2 \vec{v}_1 \cdot \vec{v}_2 - \\
& \frac{10}{3} \hat{n} \times \vec{S}_1 \cdot \vec{v}_2 \hat{n} \cdot \vec{a}_2 \vec{v}_1 \cdot \vec{v}_2 - \frac{8}{3} \hat{n} \times \vec{a}_2 \cdot \vec{S}_1 \hat{n} \cdot \vec{v}_1 \vec{v}_1 \cdot \vec{v}_2 - \frac{4}{3} \vec{S}_1 \times \vec{v}_1 \cdot \vec{v}_2 \vec{v}_2 \cdot \vec{v}_2 + \frac{2}{3} \vec{a}_1 \times \vec{S}_1 \cdot \vec{v}_2 \vec{v}_2 \cdot \vec{v}_2 + \\
& \left. \vec{a}_2 \times \vec{S}_1 \cdot \vec{v}_1 \vec{v}_2 \cdot \vec{v}_2 - \frac{4}{3} \hat{n} \times \vec{S}_1 \cdot \vec{v}_2 \hat{n} \cdot \vec{a}_1 \vec{v}_2 \cdot \vec{v}_2 - \frac{8}{3} \hat{n} \times \vec{S}_1 \cdot \vec{v}_2 \hat{n} \cdot \vec{v}_1 \vec{v}_2 \cdot \vec{v}_2 - 2 \hat{n} \times \vec{a}_2 \cdot \vec{S}_1 \hat{n} \cdot \vec{v}_1 \vec{v}_2 \cdot \vec{v}_2 \right) m_2^2 + \\
& \frac{1}{r^3} G^2 \left( 4 \vec{S}_1 \times \vec{v}_1 \cdot \vec{v}_2 (\hat{n} \cdot \vec{v}_2)^3 + 24 \hat{n} \times \vec{S}_1 \cdot \vec{v}_2 \hat{n} \cdot \vec{v}_1 (\hat{n} \cdot \vec{v}_2)^3 - 32 \hat{n} \times \vec{S}_1 \cdot \vec{v}_2 (\hat{n} \cdot \vec{v}_1)^2 (\hat{n} \cdot \vec{v}_2)^2 - \right. \\
& \frac{32}{3} \vec{S}_1 \times \vec{v}_1 \cdot \vec{v}_2 \hat{n} \cdot \vec{v}_1 (\hat{n} \cdot \vec{v}_2)^2 + \frac{16}{3} \hat{n} \times \vec{S}_1 \cdot \vec{v}_2 \vec{v}_1 \cdot \vec{v}_1 (\hat{n} \cdot \vec{v}_2)^2 - 12 \hat{n} \times \vec{S}_1 \cdot \vec{v}_2 \vec{v}_1 \cdot \vec{v}_2 (\hat{n} \cdot \vec{v}_2)^2 + \\
& \frac{16}{3} \vec{S}_1 \times \vec{v}_1 \cdot \vec{v}_2 \vec{v}_1 \cdot \vec{v}_2 \hat{n} \cdot \vec{v}_2 + \frac{64}{3} \hat{n} \times \vec{S}_1 \cdot \vec{v}_2 \hat{n} \cdot \vec{v}_1 \vec{v}_1 \cdot \vec{v}_2 \hat{n} \cdot \vec{v}_2 - \frac{8}{3} \hat{n} \times \vec{S}_1 \cdot \vec{v}_2 (\vec{v}_1 \cdot \vec{v}_2)^2 + \\
& \left. \frac{16}{3} \hat{n} \times \vec{S}_1 \cdot \vec{v}_2 (\hat{n} \cdot \vec{v}_1)^2 \vec{v}_2 \cdot \vec{v}_2 + \frac{8}{3} \vec{S}_1 \times \vec{v}_1 \cdot \vec{v}_2 \hat{n} \cdot \vec{v}_1 \vec{v}_2 \cdot \vec{v}_2 - \frac{4}{3} \hat{n} \times \vec{S}_1 \cdot \vec{v}_2 \vec{v}_1 \cdot \vec{v}_1 \vec{v}_2 \cdot \vec{v}_2 \right) m_2^2 + \\
& G^2 \left( -\frac{2}{3} \log\left(\frac{r}{R_\theta}\right) \frac{1}{\vec{a}_2 \times \vec{S}_1 \cdot \vec{v}_2} + \frac{\frac{1}{\vec{a}_2 \times \vec{S}_1 \cdot \vec{v}_2}}{3 \in_d} + \frac{7}{9} \frac{1}{\vec{a}_2 \times \vec{S}_1 \cdot \vec{v}_2} - \frac{2}{3} \hat{n} \times \vec{S}_1 \cdot \vec{v}_2 \hat{n} \cdot \frac{1}{\vec{a}_2} - \right. \\
& \left. \frac{2}{3} \hat{n} \times \vec{S}_1 \cdot \vec{v}_2 \hat{n} \cdot \vec{a}_2 + \frac{2}{3} \hat{n} \times \vec{a}_2 \cdot \vec{S}_1 \hat{n} \cdot \vec{a}_2 + \frac{2}{3} \hat{n} \times \vec{a}_2 \cdot \vec{S}_1 \hat{n} \cdot \vec{v}_2 \right) m_2^2 \Big\}
\end{aligned}$$

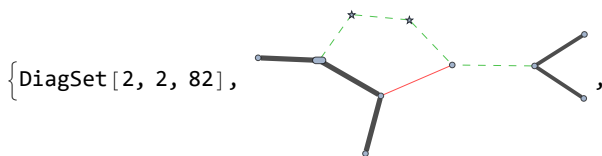

$$\begin{aligned}
& \frac{1}{r} \left( -\frac{11}{12} \hat{n} \times \vec{S}_1 \cdot \vec{v}_2 (\hat{n} \cdot \vec{a}_1)^2 - \frac{2}{3} \vec{S}_1 \times \vec{v}_1 \cdot \vec{v}_2 \hat{n} \cdot \vec{a}_1 - \frac{1}{3} \vec{S}_1 \times \vec{a}_1 \cdot \vec{v}_2 \hat{n} \cdot \vec{a}_1 + \vec{S}_1 \times \vec{v}_2 \cdot \vec{a}_2 \hat{n} \cdot \vec{a}_1 + \frac{1}{6} \hat{n} \times \vec{S}_1 \cdot \vec{v}_1 \hat{n} \cdot \vec{a}_2 \hat{n} \cdot \vec{a}_1 + \right. \\
& 2 \hat{n} \times \vec{S}_1 \cdot \vec{v}_2 \hat{n} \cdot \vec{a}_2 \hat{n} \cdot \vec{a}_1 - \frac{11}{6} \hat{n} \times \vec{S}_1 \cdot \vec{v}_2 \hat{n} \cdot \vec{v}_1 \hat{n} \cdot \vec{a}_1 - \frac{11}{6} \hat{n} \times \vec{S}_1 \cdot \vec{a}_2 \hat{n} \cdot \vec{v}_1 \hat{n} \cdot \vec{a}_1 - \frac{1}{2} \hat{n} \times \vec{S}_1 \cdot \vec{v}_1 \hat{n} \cdot \vec{v}_2 \hat{n} \cdot \vec{a}_1 - \\
& \frac{1}{6} \hat{n} \times \vec{S}_1 \cdot \vec{a}_1 \hat{n} \cdot \vec{v}_2 \hat{n} \cdot \vec{a}_1 + 4 \hat{n} \times \vec{S}_1 \cdot \vec{a}_2 \hat{n} \cdot \vec{v}_2 \hat{n} \cdot \vec{a}_1 - \frac{11}{3} \hat{n} \times \vec{S}_1 \cdot \vec{a}_2 (\hat{n} \cdot \vec{v}_1)^2 + \frac{9}{4} \hat{n} \times \vec{S}_1 \cdot \vec{v}_2 (\hat{n} \cdot \vec{v}_1)^2 - \\
& \frac{13}{12} \hat{n} \times \vec{S}_1 \cdot \vec{a}_2 (\hat{n} \cdot \vec{v}_1)^2 - \frac{2}{3} \hat{n} \times \vec{S}_1 \cdot \vec{v}_1 (\hat{n} \cdot \vec{v}_2)^2 - \frac{2}{3} \hat{n} \times \vec{S}_1 \cdot \vec{v}_2 (\hat{n} \cdot \vec{v}_2)^2 + 2 \vec{S}_1 \times \vec{v}_1 \cdot \vec{v}_2 \hat{n} \cdot \vec{a}_2 + \vec{S}_1 \times \vec{a}_1 \cdot \vec{v}_2 \hat{n} \cdot \vec{a}_2 - \\
& \left. \frac{1}{3} \vec{S}_1 \times \vec{v}_1 \cdot \vec{a}_1 \hat{n} \cdot \vec{a}_2 - \frac{4}{3} \vec{S}_1 \times \vec{v}_1 \cdot \vec{a}_2 \hat{n} \cdot \vec{v}_1 + 2 \vec{S}_1 \times \vec{v}_2 \cdot \vec{a}_2 \hat{n} \cdot \vec{v}_1 + 2 \vec{S}_1 \times \vec{v}_1 \cdot \vec{v}_2 \hat{n} \cdot \vec{v}_1 - \frac{2}{3} \vec{S}_1 \times \vec{a}_1 \cdot \vec{a}_2 \hat{n} \cdot \vec{v}_1 - \right.
\end{aligned}$$

$$\begin{aligned}
& 2 \vec{S_1} \times \vec{v_1} \cdot \frac{1}{\vec{a_2}} \hat{n} \cdot \vec{v_1} - \frac{1}{6} \hat{n} \times \vec{S_1} \cdot \vec{v_1} \hat{n} \cdot \frac{1}{\vec{a_2}} \hat{n} \cdot \vec{v_1} - \frac{2}{3} \hat{n} \times \vec{S_1} \cdot \vec{v_1} \hat{n} \cdot \vec{a_2} \hat{n} \cdot \vec{v_1} + 4 \hat{n} \times \vec{S_1} \cdot \vec{v_2} \hat{n} \cdot \vec{a_2} \hat{n} \cdot \vec{v_1} - \\
& \frac{1}{2} \hat{n} \times \vec{S_1} \cdot \vec{a_1} \hat{n} \cdot \vec{a_2} \hat{n} \cdot \vec{v_1} + \frac{1}{3} \frac{1}{\vec{S_1}} \times \vec{v_1} \cdot \vec{a_1} \hat{n} \cdot \vec{v_2} + 5 \frac{1}{\vec{S_1}} \times \vec{v_1} \cdot \vec{a_2} \hat{n} \cdot \vec{v_2} - \frac{5}{3} \frac{2}{\vec{S_1}} \times \vec{v_1} \cdot \vec{v_2} \hat{n} \cdot \vec{v_2} + \frac{5}{2} \vec{S_1} \times \vec{a_1} \cdot \vec{a_2} \hat{n} \cdot \vec{v_2} + \\
& 2 \hat{n} \times \frac{1}{\vec{S_1}} \cdot \vec{v_1} \hat{n} \cdot \vec{a_2} \hat{n} \cdot \vec{v_2} + \hat{n} \times \vec{S_1} \cdot \vec{a_1} \hat{n} \cdot \vec{a_2} \hat{n} \cdot \vec{v_2} + \frac{1}{6} \hat{n} \times \frac{1}{\vec{S_1}} \cdot \vec{a_1} \hat{n} \cdot \vec{v_1} \hat{n} \cdot \vec{v_2} + 8 \hat{n} \times \frac{1}{\vec{S_1}} \cdot \vec{a_2} \hat{n} \cdot \vec{v_1} \hat{n} \cdot \vec{v_2} + \\
& \frac{1}{2} \hat{n} \times \frac{2}{\vec{S_1}} \cdot \vec{v_1} \hat{n} \cdot \vec{v_1} \hat{n} \cdot \vec{v_2} - \frac{8}{3} \hat{n} \times \frac{2}{\vec{S_1}} \cdot \vec{v_2} \hat{n} \cdot \vec{v_1} \hat{n} \cdot \vec{v_2} - \frac{5}{12} \hat{n} \times \vec{S_1} \cdot \vec{v_2} \vec{a_1} \cdot \vec{a_1} - \frac{5}{6} \hat{n} \times \vec{S_1} \cdot \vec{v_1} \vec{a_1} \cdot \vec{a_2} - \hat{n} \times \vec{S_1} \cdot \vec{v_2} \vec{a_1} \cdot \vec{a_2} - \\
& \frac{1}{2} \hat{n} \times \frac{1}{\vec{S_1}} \cdot \vec{v_1} \vec{a_1} \cdot \vec{v_2} - \frac{2}{3} \hat{n} \times \vec{S_1} \cdot \vec{a_1} \vec{a_1} \cdot \vec{v_2} - 2 \hat{n} \times \vec{S_1} \cdot \vec{a_2} \vec{a_1} \cdot \vec{v_2} + \frac{5}{6} \hat{n} \times \vec{S_1} \cdot \vec{v_1} \vec{v_1} \cdot \frac{1}{\vec{a_2}} - \frac{5}{6} \hat{n} \times \frac{1}{\vec{S_1}} \cdot \vec{v_2} \vec{v_1} \cdot \vec{a_1} - \\
& \frac{5}{6} \hat{n} \times \vec{S_1} \cdot \vec{a_2} \vec{v_1} \cdot \vec{a_1} - \frac{8}{3} \hat{n} \times \frac{1}{\vec{S_1}} \cdot \vec{v_1} \vec{v_1} \cdot \vec{a_2} - 2 \hat{n} \times \frac{1}{\vec{S_1}} \cdot \vec{v_2} \vec{v_1} \cdot \vec{a_2} - \frac{1}{2} \hat{n} \times \vec{S_1} \cdot \vec{a_1} \vec{v_1} \cdot \vec{a_2} - \frac{5}{3} \hat{n} \times \frac{1}{\vec{S_1}} \cdot \vec{a_2} \vec{v_1} \cdot \vec{v_1} - \\
& \frac{1}{4} \hat{n} \times \frac{2}{\vec{S_1}} \cdot \vec{v_2} \vec{v_1} \cdot \vec{v_1} + \frac{17}{12} \hat{n} \times \vec{S_1} \cdot \frac{1}{\vec{a_2}} \vec{v_1} \cdot \vec{v_1} - \frac{5}{6} \hat{n} \times \frac{1}{\vec{S_1}} \cdot \vec{a_1} \vec{v_1} \cdot \vec{v_2} - 4 \hat{n} \times \frac{1}{\vec{S_1}} \cdot \vec{a_2} \vec{v_1} \cdot \vec{v_2} + \frac{1}{2} \hat{n} \times \frac{2}{\vec{S_1}} \cdot \vec{v_1} \vec{v_1} \cdot \vec{v_2} + \\
& \frac{4}{3} \hat{n} \times \frac{2}{\vec{S_1}} \cdot \vec{v_2} \vec{v_1} \cdot \vec{v_2} - \hat{n} \times \frac{1}{\vec{S_1}} \cdot \vec{v_1} \vec{v_2} \cdot \vec{a_2} - \frac{1}{2} \hat{n} \times \vec{S_1} \cdot \vec{a_1} \vec{v_2} \cdot \vec{a_2} + \frac{1}{3} \hat{n} \times \frac{2}{\vec{S_1}} \cdot \vec{v_1} \vec{v_2} \cdot \vec{v_2} + \frac{1}{3} \hat{n} \times \frac{2}{\vec{S_1}} \cdot \vec{v_2} \vec{v_2} \cdot \vec{v_2} \Big) m_1 m_2 G^2 + \\
& \frac{1}{\rho^2} \left( \frac{16}{3} \hat{n} \times \frac{1}{\vec{S_1}} \cdot \vec{v_2} (\hat{n} \cdot \vec{v_1})^3 + 2 \hat{n} \times \vec{S_1} \cdot \vec{a_2} (\hat{n} \cdot \vec{v_1})^3 - \frac{1}{4} \vec{S_1} \times \vec{a_1} \cdot \vec{v_2} (\hat{n} \cdot \vec{v_1})^2 + \frac{19}{6} \vec{S_1} \times \vec{v_1} \cdot \vec{a_2} (\hat{n} \cdot \vec{v_1})^2 - \right. \\
& \frac{13}{12} \vec{S_1} \times \vec{v_2} \cdot \vec{a_2} (\hat{n} \cdot \vec{v_1})^2 + \frac{11}{3} \hat{n} \times \vec{S_1} \cdot \vec{v_2} \hat{n} \cdot \vec{a_1} (\hat{n} \cdot \vec{v_1})^2 + \frac{1}{3} \hat{n} \times \vec{S_1} \cdot \vec{v_1} \hat{n} \cdot \vec{a_2} (\hat{n} \cdot \vec{v_1})^2 - \\
& \frac{13}{3} \hat{n} \times \vec{S_1} \cdot \vec{v_2} \hat{n} \cdot \vec{a_2} (\hat{n} \cdot \vec{v_1})^2 + \hat{n} \times \frac{1}{\vec{S_1}} \cdot \vec{v_1} \hat{n} \cdot \vec{v_2} (\hat{n} \cdot \vec{v_1})^2 - \frac{44}{3} \hat{n} \times \frac{1}{\vec{S_1}} \cdot \vec{v_2} \hat{n} \cdot \vec{v_2} (\hat{n} \cdot \vec{v_1})^2 + \\
& \frac{2}{3} \hat{n} \times \vec{S_1} \cdot \vec{a_1} \hat{n} \cdot \vec{v_2} (\hat{n} \cdot \vec{v_1})^2 - \frac{26}{3} \hat{n} \times \vec{S_1} \cdot \vec{a_2} \hat{n} \cdot \vec{v_2} (\hat{n} \cdot \vec{v_1})^2 - \frac{8}{3} \hat{n} \times \frac{1}{\vec{S_1}} \cdot \vec{v_1} (\hat{n} \cdot \vec{v_2})^2 \hat{n} \cdot \vec{v_1} + \\
& 16 \hat{n} \times \frac{1}{\vec{S_1}} \cdot \vec{v_2} (\hat{n} \cdot \vec{v_2})^2 \hat{n} \cdot \vec{v_1} - 2 \hat{n} \times \vec{S_1} \cdot \vec{a_1} (\hat{n} \cdot \vec{v_2})^2 \hat{n} \cdot \vec{v_1} + \frac{11}{6} \vec{S_1} \times \vec{v_1} \cdot \vec{v_2} \hat{n} \cdot \vec{a_1} \hat{n} \cdot \vec{v_1} - \frac{11}{3} \vec{S_1} \times \vec{v_1} \cdot \vec{v_2} \hat{n} \cdot \vec{a_2} \hat{n} \cdot \vec{v_1} - \\
& 2 \frac{1}{\vec{S_1}} \times \vec{v_1} \cdot \vec{v_2} \hat{n} \cdot \vec{v_2} \hat{n} \cdot \vec{v_1} - \frac{5}{6} \vec{S_1} \times \vec{a_1} \cdot \vec{v_2} \hat{n} \cdot \vec{v_2} \hat{n} \cdot \vec{v_1} + \frac{1}{3} \vec{S_1} \times \vec{v_1} \cdot \vec{a_1} \hat{n} \cdot \vec{v_2} \hat{n} \cdot \vec{v_1} - \frac{47}{6} \vec{S_1} \times \vec{v_1} \cdot \vec{a_2} \hat{n} \cdot \vec{v_2} \hat{n} \cdot \vec{v_1} - \\
& \frac{22}{3} \hat{n} \times \vec{S_1} \cdot \vec{v_2} \hat{n} \cdot \vec{a_1} \hat{n} \cdot \vec{v_2} \hat{n} \cdot \vec{v_1} - 2 \hat{n} \times \vec{S_1} \cdot \vec{v_1} \hat{n} \cdot \vec{a_2} \hat{n} \cdot \vec{v_2} \hat{n} \cdot \vec{v_1} + \frac{3}{2} \hat{n} \times \vec{S_1} \cdot \vec{v_1} \vec{a_1} \cdot \vec{v_2} \hat{n} \cdot \vec{v_1} + \\
& \frac{11}{6} \hat{n} \times \vec{S_1} \cdot \vec{v_2} \vec{a_1} \cdot \vec{v_2} \hat{n} \cdot \vec{v_1} + \frac{5}{3} \hat{n} \times \vec{S_1} \cdot \vec{v_2} \vec{v_1} \cdot \vec{a_1} \hat{n} \cdot \vec{v_1} - \frac{5}{3} \hat{n} \times \vec{S_1} \cdot \vec{v_1} \vec{v_1} \cdot \vec{a_2} \hat{n} \cdot \vec{v_1} + \frac{13}{6} \hat{n} \times \vec{S_1} \cdot \vec{v_2} \vec{v_1} \cdot \vec{a_2} \hat{n} \cdot \vec{v_1} - \\
& 2 \hat{n} \times \vec{S_1} \cdot \vec{a_2} \vec{v_1} \cdot \vec{v_1} \hat{n} \cdot \vec{v_1} + 4 \hat{n} \times \frac{1}{\vec{S_1}} \cdot \vec{v_1} \vec{v_1} \cdot \vec{v_2} \hat{n} \cdot \vec{v_1} + \frac{22}{3} \hat{n} \times \frac{1}{\vec{S_1}} \cdot \vec{v_2} \vec{v_1} \cdot \vec{v_2} \hat{n} \cdot \vec{v_1} + \frac{7}{6} \hat{n} \times \vec{S_1} \cdot \vec{a_1} \vec{v_1} \cdot \vec{v_2} \hat{n} \cdot \vec{v_1} + \\
& \frac{13}{3} \hat{n} \times \vec{S_1} \cdot \vec{a_2} \vec{v_1} \cdot \vec{v_2} \hat{n} \cdot \vec{v_1} + \frac{1}{2} \hat{n} \times \vec{S_1} \cdot \vec{v_1} \vec{v_2} \cdot \vec{a_2} \hat{n} \cdot \vec{v_1} + \frac{2}{3} \hat{n} \times \frac{1}{\vec{S_1}} \cdot \vec{v_1} \vec{v_2} \cdot \vec{v_2} \hat{n} \cdot \vec{v_1} - 4 \hat{n} \times \frac{1}{\vec{S_1}} \cdot \vec{v_2} \vec{v_2}$$

$$\begin{aligned}
& 2 \hat{n} \times \vec{S}_1 \cdot \vec{v}_1 \hat{n} \cdot \vec{a}_2 \vec{v}_1 \cdot \vec{v}_2 - \frac{14}{3} \hat{n} \times \vec{S}_1 \cdot \vec{v}_1 \hat{n} \cdot \vec{v}_2 \vec{v}_1 \cdot \vec{v}_2 - 8 \hat{n} \times \vec{S}_1 \cdot \vec{v}_2 \hat{n} \cdot \vec{v}_2 \vec{v}_1 \cdot \vec{v}_2 - \frac{1}{2} \hat{n} \times \vec{S}_1 \cdot \vec{a}_1 \hat{n} \cdot \vec{v}_2 \vec{v}_1 \cdot \vec{v}_2 - \\
& 2 \vec{S}_1 \times \vec{v}_1 \cdot \vec{v}_2 \vec{v}_2 \cdot \vec{v}_2 - \vec{S}_1 \times \vec{a}_1 \cdot \vec{v}_2 \vec{v}_2 \cdot \vec{v}_2 + \frac{1}{3} \vec{S}_1 \times \vec{v}_1 \cdot \vec{a}_1 \vec{v}_2 \cdot \vec{v}_2 - \frac{1}{6} \hat{n} \times \vec{S}_1 \cdot \vec{v}_1 \hat{n} \cdot \vec{a}_1 \vec{v}_2 \cdot \vec{v}_2 - \\
& 2 \hat{n} \times \vec{S}_1 \cdot \vec{v}_2 \hat{n} \cdot \vec{a}_1 \vec{v}_2 \cdot \vec{v}_2 - 2 \hat{n} \times \vec{S}_1 \cdot \vec{v}_1 \hat{n} \cdot \vec{v}_2 \vec{v}_2 \cdot \vec{v}_2 - \hat{n} \times \vec{S}_1 \cdot \vec{a}_1 \hat{n} \cdot \vec{v}_2 \vec{v}_2 \cdot \vec{v}_2 \Big) m_1 m_2 G^2 + \frac{1}{r^3} \\
& \left( -\frac{23}{8} \hat{n} \times \vec{S}_1 \cdot \vec{v}_2 (\hat{n} \cdot \vec{v}_1)^4 - \frac{13}{3} \vec{S}_1 \times \vec{v}_1 \cdot \vec{v}_2 (\hat{n} \cdot \vec{v}_1)^3 - \frac{1}{2} \hat{n} \times \vec{S}_1 \cdot \vec{v}_1 \hat{n} \cdot \vec{v}_2 (\hat{n} \cdot \vec{v}_1)^3 + 12 \hat{n} \times \vec{S}_1 \cdot \vec{v}_2 \hat{n} \cdot \vec{v}_2 (\hat{n} \cdot \vec{v}_1)^3 + \right. \\
& 2 \hat{n} \times \vec{S}_1 \cdot \vec{v}_1 (\hat{n} \cdot \vec{v}_2)^2 (\hat{n} \cdot \vec{v}_1)^2 - 26 \hat{n} \times \vec{S}_1 \cdot \vec{v}_2 (\hat{n} \cdot \vec{v}_2)^2 (\hat{n} \cdot \vec{v}_1)^2 + \frac{37}{3} \vec{S}_1 \times \vec{v}_1 \cdot \vec{v}_2 \hat{n} \cdot \vec{v}_2 (\hat{n} \cdot \vec{v}_1)^2 + \\
& \frac{17}{4} \hat{n} \times \vec{S}_1 \cdot \vec{v}_2 \vec{v}_1 \cdot \vec{v}_1 (\hat{n} \cdot \vec{v}_1)^2 + \frac{5}{2} \hat{n} \times \vec{S}_1 \cdot \vec{v}_1 \vec{v}_1 \cdot \vec{v}_2 (\hat{n} \cdot \vec{v}_1)^2 - 6 \hat{n} \times \vec{S}_1 \cdot \vec{v}_2 \vec{v}_1 \cdot \vec{v}_2 (\hat{n} \cdot \vec{v}_1)^2 - \\
& \frac{1}{3} \hat{n} \times \vec{S}_1 \cdot \vec{v}_1 \vec{v}_2 \cdot \vec{v}_2 (\hat{n} \cdot \vec{v}_1)^2 + \frac{13}{3} \hat{n} \times \vec{S}_1 \cdot \vec{v}_2 \vec{v}_2 \cdot \vec{v}_2 (\hat{n} \cdot \vec{v}_1)^2 - 4 \hat{n} \times \vec{S}_1 \cdot \vec{v}_1 (\hat{n} \cdot \vec{v}_2)^3 \hat{n} \cdot \vec{v}_1 - \\
& \frac{44}{3} \vec{S}_1 \times \vec{v}_1 \cdot \vec{v}_2 (\hat{n} \cdot \vec{v}_2)^2 \hat{n} \cdot \vec{v}_1 + 3 \vec{S}_1 \times \vec{v}_1 \cdot \vec{v}_2 \vec{v}_1 \cdot \vec{v}_1 \hat{n} \cdot \vec{v}_1 - \frac{1}{2} \hat{n} \times \vec{S}_1 \cdot \vec{v}_1 \hat{n} \cdot \vec{v}_2 \vec{v}_1 \cdot \vec{v}_1 \hat{n} \cdot \vec{v}_1 - \\
& 8 \hat{n} \times \vec{S}_1 \cdot \vec{v}_2 \hat{n} \cdot \vec{v}_2 \vec{v}_1 \cdot \vec{v}_1 \hat{n} \cdot \vec{v}_1 - \frac{14}{3} \vec{S}_1 \times \vec{v}_1 \cdot \vec{v}_2 \vec{v}_1 \cdot \vec{v}_2 \hat{n} \cdot \vec{v}_1 - \frac{22}{3} \hat{n} \times \vec{S}_1 \cdot \vec{v}_1 \hat{n} \cdot \vec{v}_2 \vec{v}_1 \cdot \vec{v}_2 \hat{n} \cdot \vec{v}_1 + \\
& \frac{52}{3} \hat{n} \times \vec{S}_1 \cdot \vec{v}_2 \hat{n} \cdot \vec{v}_2 \vec{v}_1 \cdot \vec{v}_2 \hat{n} \cdot \vec{v}_1 + \frac{11}{3} \vec{S}_1 \times \vec{v}_1 \cdot \vec{v}_2 \vec{v}_2 \cdot \vec{v}_2 \hat{n} \cdot \vec{v}_1 + 2 \hat{n} \times \vec{S}_1 \cdot \vec{v}_1 \hat{n} \cdot \vec{v}_2 \vec{v}_2 \cdot \vec{v}_2 \hat{n} \cdot \vec{v}_1 - \\
& \frac{3}{8} \hat{n} \times \vec{S}_1 \cdot \vec{v}_2 (\vec{v}_1 \cdot \vec{v}_1)^2 + \frac{5}{3} \hat{n} \times \vec{S}_1 \cdot \vec{v}_1 (\vec{v}_1 \cdot \vec{v}_2)^2 - \frac{13}{6} \hat{n} \times \vec{S}_1 \cdot \vec{v}_2 (\vec{v}_1 \cdot \vec{v}_2)^2 + \frac{8}{3} \hat{n} \times \vec{S}_1 \cdot \vec{v}_1 (\hat{n} \cdot \vec{v}_2)^2 \vec{v}_1 \cdot \vec{v}_1 + \\
& \frac{34}{3} \hat{n} \times \vec{S}_1 \cdot \vec{v}_2 (\hat{n} \cdot \vec{v}_2)^2 \vec{v}_1 \cdot \vec{v}_1 - \frac{13}{3} \vec{S}_1 \times \vec{v}_1 \cdot \vec{v}_2 \hat{n} \cdot \vec{v}_2 \vec{v}_1 \cdot \vec{v}_1 + 8 \hat{n} \times \vec{S}_1 \cdot \vec{v}_1 (\hat{n} \cdot \vec{v}_2)^2 \vec{v}_1 \cdot \vec{v}_2 + \\
& \frac{13}{3} \vec{S}_1 \times \vec{v}_1 \cdot \vec{v}_2 \hat{n} \cdot \vec{v}_2 \vec{v}_1 \cdot \vec{v}_2 + \frac{1}{2} \hat{n} \times \vec{S}_1 \cdot \vec{v}_1 \vec{v}_1 \cdot \vec{v}_1 \vec{v}_1 \cdot \vec{v}_2 + 2 \hat{n} \times \vec{S}_1 \cdot \vec{v}_2 \vec{v}_1 \cdot \vec{v}_1 \vec{v}_1 \cdot \vec{v}_2 - \\
& \frac{2}{3} \hat{n} \times \vec{S}_1 \cdot \vec{v}_1 \vec{v}_1 \cdot \vec{v}_1 \vec{v}_2 \cdot \vec{v}_2 - \frac{17}{6} \hat{n} \times \vec{S}_1 \cdot \vec{v}_2 \vec{v}_1 \cdot \vec{v}_1 \vec{v}_2 \cdot \vec{v}_2 - 2 \hat{n} \times \vec{S}_1 \cdot \vec{v}_1 \vec{v}_1 \cdot \vec{v}_2 \vec{v}_2 \cdot \vec{v}_2 \Big) m_1 m_2 G^2 + \\
& r m_1 m_2 \left( \frac{1}{3} \log\left(\frac{r}{R_\theta}\right) \hat{n} \times \vec{S}_1 \cdot \vec{a}_2 - \frac{\hat{n} \times \vec{S}_1 \cdot \vec{a}_2}{6 \epsilon_d} + \frac{7}{9} \hat{n} \times \vec{S}_1 \cdot \vec{a}_2 \right) G^2 + \\
& m_1 m_2 \left( -\frac{8}{3} \log\left(\frac{r}{R_\theta}\right) \vec{S}_1 \times \vec{v}_1 \cdot \vec{a}_2 + \frac{1}{9} \vec{S}_1 \times \vec{v}_1 \cdot \vec{a}_2 - \frac{5}{6} \vec{S}_1 \times \vec{a}_1 \cdot \vec{v}_2 - \frac{5}{3} \vec{S}_1 \times \vec{v}_1 \cdot \vec{a}_2 + \frac{7}{9} \vec{S}_1 \times \vec{v}_2 \cdot \vec{a}_2 + \right. \\
& \frac{1}{18} \vec{S}_1 \times \vec{a}_1 \cdot \vec{a}_2 + \frac{1}{3} \hat{n} \times \vec{S}_1 \cdot \vec{v}_1 \hat{n} \cdot \vec{a}_2 + \frac{1}{6} \hat{n} \times \vec{S}_1 \cdot \vec{a}_1 \hat{n} \cdot \vec{a}_2 - \frac{2}{3} \hat{n} \times \vec{S}_1 \cdot \vec{v}_2 \hat{n} \cdot \vec{a}_1 + \hat{n} \times \vec{S}_1 \cdot \vec{a}_2 \hat{n} \cdot \vec{a}_1 - \\
& \frac{1}{3} \hat{n} \times \vec{S}_1 \cdot \vec{v}_1 \hat{n} \cdot \vec{a}_2 - \frac{1}{3} \hat{n} \times \vec{S}_1 \cdot \vec{v}_2 \hat{n} \cdot \vec{a}_2 + 2 \hat{n} \times \vec{S}_1 \cdot \vec{a}_2 \hat{n} \cdot \vec{v}_1 - \frac{4}{3} \hat{n} \times \vec{S}_1 \cdot \vec{a}_2 \hat{n} \cdot \vec{v}_1 - \frac{1}{6} \hat{n} \times \vec{S}_1 \cdot \vec{a}_1 \hat{n} \cdot \vec{v}_2 - \\
& \frac{2}{3} \hat{n} \times \vec{S}_1 \cdot \vec{a}_2 \hat{n} \cdot \vec{v}_2 + \vec{S}_1 \times \vec{a}_1 \cdot \vec{v}_2 \log\left(\frac{r}{R_\theta}\right) + 2 \vec{S}_1 \times \vec{v}_1 \cdot \vec{a}_2 \log\left(\frac{r}{R_\theta}\right) + \frac{1}{3} \vec{S}_1 \times \vec{v}_2 \cdot \vec{a}_2 \log\left(\frac{r}{R_\theta}\right) - \\
& \left. \frac{4}{3} \vec{S}_1 \times \vec{a}_1 \cdot \vec{a}_2 \log\left(\frac{r}{R_\theta}\right) + \frac{\frac{4}{3} \vec{S}_1 \times \vec{v}_1 \cdot \vec{a}_2 - \frac{1}{2} \vec{S}_1 \times \vec{a}_1 \cdot \vec{v}_2 - \vec{S}_1 \times \vec{v}_1 \cdot \vec{a}_2 - \frac{1}{6} \vec{S}_1 \times \vec{v}_2 \cdot \vec{a}_2 + \frac{2}{3} \vec{S}_1 \times \vec{a}_1 \cdot \vec{a}_2}{\epsilon_d} \right) G^2 \Big\}
\end{aligned}$$

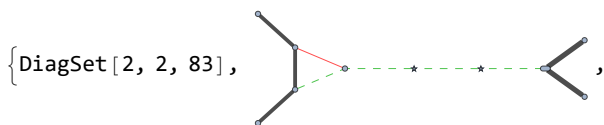

$$\frac{1}{r} G^2 \left( \frac{8}{3} \hat{n} \times \vec{a}_2 \cdot \vec{S}_1 (\hat{n} \cdot \vec{v}_1)^2 - \frac{8}{3} \vec{a}_2 \times \vec{S}_1 \cdot \vec{v}_1 \hat{n} \cdot \vec{v}_1 + \frac{8}{3} \vec{a}_2 \times \vec{S}_1 \cdot \vec{v}_2 \hat{n} \cdot \vec{v}_1 + \right.$$



$$\begin{aligned}
& \frac{16}{3} \hat{n} \times \vec{S}_1 \cdot \vec{v}_2 \hat{n} \cdot \vec{a}_2 \hat{n} \cdot \vec{v}_1 - \frac{32}{3} \hat{n} \times \vec{a}_2 \cdot \vec{S}_1 \hat{n} \cdot \vec{v}_2 \hat{n} \cdot \vec{v}_1 - \frac{8}{3} \hat{n} \times \vec{S}_1 \cdot \vec{v}_2 (\hat{n} \cdot \vec{v}_2)^2 + \frac{4}{3} \vec{a}_2 \times \vec{S}_1 \cdot \vec{v}_2 \hat{n} \cdot \vec{a}_1 + \\
& \frac{8}{3} \vec{S}_1 \times \vec{v}_1 \cdot \vec{v}_2 \hat{n} \cdot \vec{a}_2 - \frac{4}{3} \vec{a}_1 \times \vec{S}_1 \cdot \vec{v}_2 \hat{n} \cdot \vec{a}_2 + \frac{8}{3} \hat{n} \times \vec{S}_1 \cdot \vec{v}_2 \hat{n} \cdot \vec{a}_1 \hat{n} \cdot \vec{a}_2 + \frac{8}{3} \vec{a}_1 \times \vec{a}_2 \cdot \vec{S}_1 \hat{n} \cdot \vec{v}_2 + \\
& \frac{16}{3} \vec{a}_2 \times \vec{S}_1 \cdot \vec{v}_1 \hat{n} \cdot \vec{v}_2 - \frac{16}{3} \hat{n} \times \vec{a}_2 \cdot \vec{S}_1 \hat{n} \cdot \vec{a}_1 \hat{n} \cdot \vec{v}_2 - \frac{4}{3} \hat{n} \times \vec{S}_1 \cdot \vec{v}_2 \vec{a}_1 \cdot \vec{a}_2 + \frac{8}{3} \hat{n} \times \vec{a}_2 \cdot \vec{S}_1 \vec{a}_1 \cdot \vec{v}_2 - \\
& \frac{8}{3} \hat{n} \times \vec{S}_1 \cdot \vec{v}_2 \vec{a}_2 \cdot \vec{v}_1 - \frac{4}{3} \hat{n} \times \vec{a}_2 \cdot \vec{S}_1 \vec{v}_1 \cdot \vec{v}_1 + \frac{16}{3} \hat{n} \times \vec{a}_2 \cdot \vec{S}_1 \vec{v}_1 \cdot \vec{v}_2 + \frac{4}{3} \hat{n} \times \vec{S}_1 \cdot \vec{v}_2 \vec{v}_2 \cdot \vec{v}_2 \Big) m_2^2 + \\
& \frac{1}{r^2} G^2 \left( -\frac{8}{3} \vec{a}_2 \times \vec{S}_1 \cdot \vec{v}_2 (\hat{n} \cdot \vec{v}_1)^2 - \frac{32}{3} \hat{n} \times \vec{S}_1 \cdot \vec{v}_2 \hat{n} \cdot \vec{a}_2 (\hat{n} \cdot \vec{v}_1)^2 + \frac{64}{3} \hat{n} \times \vec{a}_2 \cdot \vec{S}_1 \hat{n} \cdot \vec{v}_2 (\hat{n} \cdot \vec{v}_1)^2 + \right. \\
& \frac{64}{3} \hat{n} \times \vec{S}_1 \cdot \vec{v}_2 (\hat{n} \cdot \vec{v}_2)^2 \hat{n} \cdot \vec{v}_1 - \frac{16}{3} \vec{S}_1 \times \vec{v}_1 \cdot \vec{v}_2 \hat{n} \cdot \vec{a}_2 \hat{n} \cdot \vec{v}_1 - \frac{32}{3} \vec{a}_2 \times \vec{S}_1 \cdot \vec{v}_1 \hat{n} \cdot \vec{v}_2 \hat{n} \cdot \vec{v}_1 + \\
& \frac{16}{3} \hat{n} \times \vec{S}_1 \cdot \vec{v}_2 \vec{a}_2 \cdot \vec{v}_1 \hat{n} \cdot \vec{v}_1 - \frac{32}{3} \hat{n} \times \vec{a}_2 \cdot \vec{S}_1 \vec{v}_1 \cdot \vec{v}_2 \hat{n} \cdot \vec{v}_1 - \frac{16}{3} \hat{n} \times \vec{S}_1 \cdot \vec{v}_2 \vec{v}_2 \cdot \vec{v}_2 \hat{n} \cdot \vec{v}_1 + \frac{16}{3} \vec{S}_1 \times \vec{v}_1 \cdot \vec{v}_2 (\hat{n} \cdot \vec{v}_2)^2 - \\
& \frac{8}{3} \vec{a}_1 \times \vec{S}_1 \cdot \vec{v}_2 (\hat{n} \cdot \vec{v}_2)^2 + \frac{32}{3} \hat{n} \times \vec{S}_1 \cdot \vec{v}_2 \hat{n} \cdot \vec{a}_1 (\hat{n} \cdot \vec{v}_2)^2 - \frac{16}{3} \hat{n} \times \vec{S}_1 \cdot \vec{v}_2 \hat{n} \cdot \vec{v}_2 \vec{a}_1 \cdot \vec{v}_2 + \frac{8}{3} \vec{S}_1 \times \vec{v}_1 \cdot \vec{v}_2 \vec{a}_2 \cdot \vec{v}_1 + \\
& \frac{4}{3} \vec{a}_2 \times \vec{S}_1 \cdot \vec{v}_2 \vec{v}_1 \cdot \vec{v}_1 + \frac{8}{3} \hat{n} \times \vec{S}_1 \cdot \vec{v}_2 \hat{n} \cdot \vec{a}_2 \vec{v}_1 \cdot \vec{v}_1 - \frac{16}{3} \hat{n} \times \vec{a}_2 \cdot \vec{S}_1 \hat{n} \cdot \vec{v}_2 \vec{v}_1 \cdot \vec{v}_1 + \frac{16}{3} \vec{a}_2 \times \vec{S}_1 \cdot \vec{v}_1 \vec{v}_1 \cdot \vec{v}_2 - \\
& \left. \frac{32}{3} \hat{n} \times \vec{S}_1 \cdot \vec{v}_2 \hat{n} \cdot \vec{v}_2 \vec{v}_1 \cdot \vec{v}_2 - \frac{8}{3} \vec{S}_1 \times \vec{v}_1 \cdot \vec{v}_2 \vec{v}_2 \cdot \vec{v}_2 + \frac{4}{3} \vec{a}_1 \times \vec{S}_1 \cdot \vec{v}_2 \vec{v}_2 \cdot \vec{v}_2 - \frac{8}{3} \hat{n} \times \vec{S}_1 \cdot \vec{v}_2 \hat{n} \cdot \vec{a}_1 \vec{v}_2 \cdot \vec{v}_2 \right) m_2^2 + \\
& \frac{1}{r^3} G^2 \left( -64 \hat{n} \times \vec{S}_1 \cdot \vec{v}_2 (\hat{n} \cdot \vec{v}_2)^2 (\hat{n} \cdot \vec{v}_1)^2 + \frac{32}{3} \hat{n} \times \vec{S}_1 \cdot \vec{v}_2 \vec{v}_2 \cdot \vec{v}_2 (\hat{n} \cdot \vec{v}_1)^2 - \frac{64}{3} \vec{S}_1 \times \vec{v}_1 \cdot \vec{v}_2 (\hat{n} \cdot \vec{v}_2)^2 \hat{n} \cdot \vec{v}_1 + \right. \\
& \frac{128}{3} \hat{n} \times \vec{S}_1 \cdot \vec{v}_2 \hat{n} \cdot \vec{v}_2 \vec{v}_1 \cdot \vec{v}_2 \hat{n} \cdot \vec{v}_1 + \frac{16}{3} \vec{S}_1 \times \vec{v}_1 \cdot \vec{v}_2 \vec{v}_2 \cdot \vec{v}_2 \hat{n} \cdot \vec{v}_1 - \frac{16}{3} \hat{n} \times \vec{S}_1 \cdot \vec{v}_2 (\vec{v}_1 \cdot \vec{v}_2)^2 + \\
& \left. \frac{32}{3} \hat{n} \times \vec{S}_1 \cdot \vec{v}_2 (\hat{n} \cdot \vec{v}_2)^2 \vec{v}_1 \cdot \vec{v}_1 + \frac{32}{3} \vec{S}_1 \times \vec{v}_1 \cdot \vec{v}_2 \hat{n} \cdot \vec{v}_2 \vec{v}_1 \cdot \vec{v}_2 - \frac{8}{3} \hat{n} \times \vec{S}_1 \cdot \vec{v}_2 \vec{v}_1 \cdot \vec{v}_1 \vec{v}_2 \cdot \vec{v}_2 \right) m_2^2 + \\
& G^2 r \left( -\frac{4}{3} \log\left(\frac{r}{R_\theta}\right) \hat{n} \times \vec{a}_2 \cdot \vec{S}_1 + \frac{2 \hat{n} \times \vec{a}_2 \cdot \vec{S}_1}{3 \epsilon_d} + \frac{8}{9} \hat{n} \times \vec{a}_2 \cdot \vec{S}_1 \right) m_2^2 + \\
& G^2 \left( -\frac{8}{3} \log\left(\frac{r}{R_\theta}\right) \vec{a}_2 \times \vec{S}_1 \cdot \vec{v}_1 + \frac{16}{9} \vec{a}_2 \times \vec{S}_1 \cdot \vec{v}_1 + \frac{8}{9} \vec{a}_1 \times \vec{a}_2 \cdot \vec{S}_1 - \frac{8}{9} \vec{a}_2 \times \vec{S}_1 \cdot \vec{v}_2 - \right. \\
& \frac{4}{3} \hat{n} \times \vec{a}_2 \cdot \vec{S}_1 \hat{n} \cdot \vec{a}_1 - \frac{4}{3} \hat{n} \times \vec{S}_1 \cdot \vec{v}_2 \hat{n} \cdot \vec{a}_2 - \frac{8}{3} \hat{n} \times \vec{a}_2 \cdot \vec{S}_1 \hat{n} \cdot \vec{v}_1 + \frac{8}{3} \hat{n} \times \vec{a}_2 \cdot \vec{S}_1 \hat{n} \cdot \vec{v}_2 - \\
& \left. \frac{4}{3} \vec{a}_1 \times \vec{a}_2 \cdot \vec{S}_1 \log\left(\frac{r}{R_\theta}\right) + \frac{4}{3} \vec{a}_2 \times \vec{S}_1 \cdot \vec{v}_2 \log\left(\frac{r}{R_\theta}\right) + \frac{\frac{4}{3} \vec{a}_2 \times \vec{S}_1 \cdot \vec{v}_1 + \frac{2}{3} \vec{a}_1 \times \vec{a}_2 \cdot \vec{S}_1 - \frac{2}{3} \vec{a}_2 \times \vec{S}_1 \cdot \vec{v}_2}{\epsilon_d} \right) m_2^2 \Big\}
\end{aligned}$$

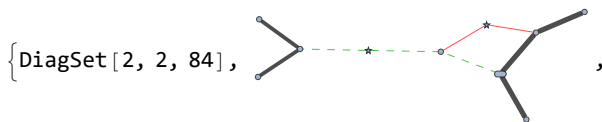

$$\begin{aligned}
& \frac{1}{r} \left( -\frac{7}{6} \hat{n} \times \vec{S}_1 \cdot \vec{a}_2 (\hat{n} \cdot \vec{v}_1)^2 - \frac{2}{3} \hat{n} \times \vec{S}_1 \cdot \vec{a}_2 (\hat{n} \cdot \vec{v}_1)^2 + \frac{1}{3} \vec{S}_1 \times \vec{v}_2 \cdot \vec{a}_2 \hat{n} \cdot \vec{v}_1 - \frac{1}{3} \vec{S}_1 \times \vec{a}_1 \cdot \vec{a}_2 \hat{n} \cdot \vec{v}_1 + \frac{1}{3} \vec{S}_1 \times \vec{v}_1 \cdot \vec{a}_2 \hat{n} \cdot \vec{v}_1 + \right. \\
& \hat{n} \times \vec{S}_1 \cdot \vec{v}_1 \hat{n} \cdot \vec{a}_2 \hat{n} \cdot \vec{v}_1 - \hat{n} \times \vec{S}_1 \cdot \vec{a}_2 \hat{n} \cdot \vec{a}_1 \hat{n} \cdot \vec{v}_1 + \frac{5}{3} \hat{n} \times \vec{S}_1 \cdot \vec{v}_1 \hat{n} \cdot \vec{a}_2 \hat{n} \cdot \vec{v}_1 + \frac{2}{3} \hat{n} \times \vec{S}_1 \cdot \vec{v}_2 \hat{n} \cdot \vec{a}_2 \hat{n} \cdot \vec{v}_1 + \\
& \frac{2}{3} \hat{n} \times \vec{S}_1 \cdot \vec{a}_1 \hat{n} \cdot \vec{a}_2 \hat{n} \cdot \vec{v}_1 + \frac{4}{3} \hat{n} \times \vec{S}_1 \cdot \vec{a}_2 \hat{n} \cdot \vec{v}_2 \hat{n} \cdot \vec{v}_1 + \frac{2}{3} \hat{n} \times \vec{S}_1 \cdot \vec{v}_2 \hat{n} \cdot \vec{v}_2 \hat{n} \cdot \vec{v}_1 - \hat{n} \times \vec{S}_1 \cdot \vec{a}_1 (\hat{n} \cdot \vec{v}_2)^2 - \\
& \left. \hat{n} \times \vec{S}_1 \cdot \vec{v}_1 (\hat{n} \cdot \vec{v}_2)^2 - \frac{1}{3} \vec{S}_1 \times \vec{v}_1 \cdot \vec{a}_2 \hat{n} \cdot \vec{a}_1 + \frac{1}{3} \vec{S}_1 \times \vec{v}_2 \cdot \vec{a}_2 \hat{n} \cdot \vec{a}_1 + \frac{1}{3} \vec{S}_1 \times \vec{v}_1 \cdot \vec{v}_2 \hat{n} \cdot \vec{a}_2 + \frac{1}{3} \vec{S}_1 \times \vec{a}_1 \cdot \vec{v}_2 \hat{n} \cdot \vec{a}_2 + \right.
\end{aligned}$$

$$\frac{1}{r^3}$$

$$\begin{aligned}
 & \frac{4}{3} \hat{n} \times \vec{S}_1 \cdot \vec{v}_2 (\vec{v}_1 \cdot \vec{v}_2)^2 + \frac{8}{3} \hat{n} \times \vec{S}_1 \cdot \vec{v}_1 (\hat{n} \cdot \vec{v}_2)^2 \vec{v}_1 \cdot \vec{v}_1 + \frac{8}{3} \hat{n} \times \vec{S}_1 \cdot \vec{v}_2 (\hat{n} \cdot \vec{v}_2)^2 \vec{v}_1 \cdot \vec{v}_1 - \\
 & \frac{1}{3} \vec{S}_1 \times \vec{v}_1 \cdot \vec{v}_2 \hat{n} \cdot \vec{v}_2 \vec{v}_1 \cdot \vec{v}_1 - 12 \hat{n} \times \vec{S}_1 \cdot \vec{v}_1 (\hat{n} \cdot \vec{v}_2)^2 \vec{v}_1 \cdot \vec{v}_2 + \frac{8}{3} \vec{S}_1 \times \vec{v}_1 \cdot \vec{v}_2 \hat{n} \cdot \vec{v}_2 \vec{v}_1 \cdot \vec{v}_2 - \\
 & \frac{2}{3} \hat{n} \times \vec{S}_1 \cdot \vec{v}_1 \vec{v}_1 \cdot \vec{v}_1 \vec{v}_2 \cdot \vec{v}_2 - \frac{2}{3} \hat{n} \times \vec{S}_1 \cdot \vec{v}_2 \vec{v}_1 \cdot \vec{v}_1 \vec{v}_2 \cdot \vec{v}_2 + 3 \hat{n} \times \vec{S}_1 \cdot \vec{v}_1 \vec{v}_1 \cdot \vec{v}_2 \vec{v}_2 \cdot \vec{v}_2 \Big) m_1 m_2 G^2 + \\
 & m_1 m_2 \left( \frac{2}{3} \log \left( \frac{r}{R_\theta} \right) \frac{1}{\vec{S}_1 \times \vec{a}_1 \cdot \vec{a}_2} - \frac{5}{18} \frac{1}{\vec{S}_1 \times \vec{a}_1 \cdot \vec{a}_2} - \frac{5}{18} \frac{1}{\vec{S}_1 \times \vec{v}_1 \cdot \vec{a}_2} - \frac{5}{18} \frac{2}{\vec{S}_1 \times \vec{v}_1 \cdot \vec{a}_2} - \frac{5}{18} \frac{1}{\vec{S}_1 \times \vec{a}_1 \cdot \vec{a}_2} - \right. \\
 & \frac{1}{2} \hat{n} \times \vec{S}_1 \cdot \vec{v}_1 \hat{n} \cdot \vec{a}_2 - \frac{1}{2} \hat{n} \times \vec{S}_1 \cdot \vec{a}_1 \hat{n} \cdot \vec{a}_2 + \frac{1}{3} \hat{n} \times \vec{S}_1 \cdot \vec{a}_2 \hat{n} \cdot \vec{a}_1 + \frac{1}{3} \hat{n} \times \vec{S}_1 \cdot \vec{a}_2 \hat{n} \cdot \vec{a}_1 - \frac{1}{2} \hat{n} \times \vec{S}_1 \cdot \vec{a}_1 \hat{n} \cdot \vec{a}_2 - \\
 & \frac{1}{2} \hat{n} \times \vec{S}_1 \cdot \vec{v}_1 \hat{n} \cdot \vec{a}_2 + \frac{1}{3} \hat{n} \times \vec{S}_1 \cdot \vec{a}_2 \hat{n} \cdot \vec{v}_1 + \frac{1}{3} \hat{n} \times \vec{S}_1 \cdot \vec{a}_2 \hat{n} \cdot \vec{v}_1 + \frac{2}{3} \frac{1}{\vec{S}_1 \times \vec{v}_1 \cdot \vec{a}_2} \log \left( \frac{r}{R_\theta} \right) + \frac{2}{3} \frac{2}{\vec{S}_1 \times \vec{v}_1 \cdot \vec{a}_2} \log \left( \frac{r}{R_\theta} \right) + \\
 & \left. \frac{2}{3} \vec{S}_1 \times \vec{a}_1 \cdot \vec{a}_2 \log \left( \frac{r}{R_\theta} \right) + \frac{-\frac{1}{3} \vec{S}_1 \times \vec{a}_1 \cdot \vec{a}_2 - \frac{1}{3} \vec{S}_1 \times \vec{v}_1 \cdot \vec{a}_2 - \frac{1}{3} \vec{S}_1 \times \vec{v}_1 \cdot \vec{a}_2 - \frac{1}{3} \vec{S}_1 \times \vec{a}_1 \cdot \vec{a}_2}{\epsilon_d} \right) G^2 \Big\}
 \end{aligned}$$

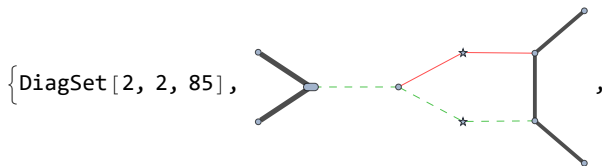

$$\begin{aligned}
 & \frac{1}{r} G^2 \left( -\frac{2}{3} \hat{n} \times \vec{S}_1 \cdot \vec{v}_2 (\hat{n} \cdot \vec{a}_2)^2 + \frac{4}{3} \frac{1}{\vec{S}_1 \times \vec{v}_1 \cdot \vec{v}_2} \hat{n} \cdot \vec{a}_2 - \frac{2}{3} \vec{a}_1 \times \vec{S}_1 \cdot \vec{v}_2 \hat{n} \cdot \vec{a}_2 + 2 \vec{a}_2 \times \vec{S}_1 \cdot \vec{v}_1 \hat{n} \cdot \vec{a}_2 - \right. \\
 & 2 \vec{a}_2 \times \vec{S}_1 \cdot \vec{v}_2 \hat{n} \cdot \vec{a}_2 + \frac{4}{3} \hat{n} \times \vec{S}_1 \cdot \vec{v}_2 \hat{n} \cdot \vec{a}_1 \hat{n} \cdot \vec{a}_2 + \frac{8}{3} \hat{n} \times \vec{S}_1 \cdot \vec{v}_2 \hat{n} \cdot \vec{v}_1 \hat{n} \cdot \vec{a}_2 - 4 \hat{n} \times \vec{a}_2 \cdot \vec{S}_1 \hat{n} \cdot \vec{v}_1 \hat{n} \cdot \vec{a}_2 - \\
 & \frac{16}{3} \hat{n} \times \vec{S}_1 \cdot \vec{v}_2 \hat{n} \cdot \vec{v}_2 \hat{n} \cdot \vec{a}_2 + \frac{16}{3} \hat{n} \times \vec{a}_2 \cdot \vec{S}_1 \hat{n} \cdot \vec{v}_2 \hat{n} \cdot \vec{a}_2 + \frac{2}{3} \hat{n} \times \vec{a}_2 \cdot \vec{S}_1 (\hat{n} \cdot \vec{v}_2)^2 - 2 \hat{n} \times \vec{S}_1 \cdot \vec{v}_2 (\hat{n} \cdot \vec{v}_2)^2 + \\
 & \frac{14}{3} \hat{n} \times \vec{a}_2 \cdot \vec{S}_1 (\hat{n} \cdot \vec{v}_2)^2 + \frac{2}{3} \vec{S}_1 \times \vec{v}_1 \cdot \vec{v}_2 \hat{n} \cdot \vec{a}_2 + \frac{2}{3} \vec{a}_2 \times \vec{S}_1 \cdot \vec{v}_2 \hat{n} \cdot \vec{a}_1 + \frac{2}{3} \frac{1}{\vec{a}_2 \times \vec{S}_1 \cdot \vec{v}_2} \hat{n} \cdot \vec{v}_1 + \frac{4}{3} \vec{a}_2 \times \vec{S}_1 \cdot \vec{v}_2 \hat{n} \cdot \vec{v}_1 + \\
 & \frac{4}{3} \hat{n} \times \vec{S}_1 \cdot \vec{v}_2 \hat{n} \cdot \vec{a}_2 \hat{n} \cdot \vec{v}_1 + \frac{4}{3} \frac{1}{\vec{a}_2 \times \vec{S}_1 \cdot \vec{v}_1} \hat{n} \cdot \vec{v}_2 + \frac{4}{3} \vec{a}_1 \times \vec{a}_2 \cdot \vec{S}_1 \hat{n} \cdot \vec{v}_2 + \frac{8}{3} \vec{a}_2 \times \vec{S}_1 \cdot \vec{v}_1 \hat{n} \cdot \vec{v}_2 - \\
 & 2 \vec{a}_2 \times \vec{S}_1 \cdot \vec{v}_2 \hat{n} \cdot \vec{v}_2 - \frac{4}{3} \hat{n} \times \vec{S}_1 \cdot \vec{v}_2 \hat{n} \cdot \vec{a}_2 \hat{n} \cdot \vec{v}_2 - \frac{8}{3} \hat{n} \times \vec{a}_2 \cdot \vec{S}_1 \hat{n} \cdot \vec{a}_1 \hat{n} \cdot \vec{v}_2 - \frac{8}{3} \hat{n} \times \vec{a}_2 \cdot \vec{S}_1 \hat{n} \cdot \vec{v}_1 \hat{n} \cdot \vec{v}_2 - \\
 & \frac{16}{3} \hat{n} \times \vec{a}_2 \cdot \vec{S}_1 \hat{n} \cdot \vec{v}_1 \hat{n} \cdot \vec{v}_2 - \frac{2}{3} \hat{n} \times \vec{S}_1 \cdot \vec{v}_2 \vec{a}_2 \cdot \vec{v}_1 + \frac{2}{3} \hat{n} \times \vec{S}_1 \cdot \vec{v}_2 \vec{a}_2 \cdot \vec{v}_2 - \frac{2}{3} \hat{n} \times \vec{S}_1 \cdot \vec{v}_2 \vec{a}_1 \cdot \vec{a}_2 + \\
 & \frac{4}{3} \hat{n} \times \vec{a}_2 \cdot \vec{S}_1 \vec{a}_1 \cdot \vec{v}_2 - \frac{2}{3} \hat{n} \times \vec{S}_1 \cdot \vec{v}_2 \vec{a}_2 \cdot \vec{a}_2 - \frac{4}{3} \hat{n} \times \vec{S}_1 \cdot \vec{v}_2 \vec{a}_2 \cdot \vec{v}_1 + 2 \hat{n} \times \vec{a}_2 \cdot \vec{S}_1 \vec{a}_2 \cdot \vec{v}_1 + \frac{2}{3} \hat{n} \times \vec{S}_1 \cdot \vec{v}_2 \vec{a}_2 \cdot \vec{v}_2 - \\
 & \frac{2}{3} \hat{n} \times \vec{a}_2 \cdot \vec{S}_1 \vec{a}_2 \cdot \vec{v}_2 + \frac{4}{3} \hat{n} \times \vec{a}_2 \cdot \vec{S}_1 \vec{v}_1 \cdot \vec{v}_2 + \frac{8}{3} \hat{n} \times \vec{a}_2 \cdot \vec{S}_1 \vec{v}_1 \cdot \vec{v}_2 - \frac{4}{3} \hat{n} \times \vec{a}_2 \cdot \vec{S}_1 \vec{v}_2 \cdot \vec{v}_2 - \frac{4}{3} \hat{n} \times \vec{a}_2 \cdot \vec{S}_1 \vec{v}_2 \cdot \vec{v}_2 \Big) m_2^2 + \\
 & \frac{1}{r^2} G^2 \left( -8 \hat{n} \times \vec{S}_1 \cdot \vec{v}_2 (\hat{n} \cdot \vec{v}_2)^3 + \frac{16}{3} \hat{n} \times \vec{a}_2 \cdot \vec{S}_1 (\hat{n} \cdot \vec{v}_2)^3 + 4 \frac{1}{\vec{S}_1 \times \vec{v}_1 \cdot \vec{v}_2} (\hat{n} \cdot \vec{v}_2)^2 - 2 \vec{a}_1 \times \vec{S}_1 \cdot \vec{v}_2 (\hat{n} \cdot \vec{v}_2)^2 + \right. \\
 & \frac{14}{3} \vec{a}_2 \times \vec{S}_1 \cdot \vec{v}_1 (\hat{n} \cdot \vec{v}_2)^2 - \frac{7}{3} \vec{a}_2 \times \vec{S}_1 \cdot \vec{v}_2 (\hat{n} \cdot \vec{v}_2)^2 + 8 \hat{n} \times \vec{S}_1 \cdot \vec{v}_2 \hat{n} \cdot \vec{a}_1 (\hat{n} \cdot \vec{v}_2)^2 - \\
 & \frac{20}{3} \hat{n} \times \vec{S}_1 \cdot \vec{v}_2 \hat{n} \cdot \vec{a}_2 (\hat{n} \cdot \vec{v}_2)^2 + 16 \hat{n} \times \vec{S}_1 \cdot \vec{v}_2 \hat{n} \cdot \vec{v}_1 (\hat{n} \cdot \vec{v}_2)^2 - \frac{56}{3} \hat{n} \times \vec{a}_2 \cdot \vec{S}_1 \hat{n} \cdot \vec{v}_1 (\hat{n} \cdot \vec{v}_2)^2 + \\
 & \frac{32}{3} \hat{n} \times \vec{a}_2 \cdot \vec{S}_1 (\hat{n} \cdot \vec{v}_1)^2 \hat{n} \cdot \vec{v}_2 + \frac{16}{3} \vec{S}_1 \times \vec{v}_1 \cdot \vec{v}_2 \hat{n} \cdot \vec{a}_2 \hat{n} \cdot \vec{v}_2 - \frac{16}{3} \vec{a}_2 \times \vec{S}_1 \cdot \vec{v}_1 \hat{n} \cdot \vec{v}_1 \hat{n} \cdot \vec{v}_2 + \\
 & \left. 4 \vec{a}_2 \times \vec{S}_1 \cdot \vec{v}_2 \hat{n} \cdot \vec{v}_1 \hat{n} \cdot \vec{v}_2 + \frac{64}{3} \hat{n} \times \vec{S}_1 \cdot \vec{v}_2 \hat{n} \cdot \vec{a}_2 \hat{n} \cdot \vec{v}_1 \hat{n} \cdot \vec{v}_2 - 4 \hat{n} \times \vec{S}_1 \cdot \vec{v}_2 \vec{a}_1 \cdot \vec{v}_2 \hat{n} \cdot \vec{v}_2 - \right.
 \end{aligned}$$

$$\begin{aligned}
& \frac{16}{3} \hat{n} \times \vec{S}_1 \cdot \vec{v}_2 \vec{a}_2 \cdot \vec{v}_1 \hat{n} \cdot \vec{v}_2 - \frac{2}{3} \hat{n} \times \vec{S}_1 \cdot \vec{v}_2 \vec{a}_2 \cdot \vec{v}_2 \hat{n} \cdot \vec{v}_2 - \frac{8}{3} \hat{n} \times \vec{a}_2 \cdot \vec{S}_1 \vec{v}_1 \cdot \vec{v}_1 \hat{n} \cdot \vec{v}_2 - 8 \hat{n} \times \vec{S}_1 \cdot \vec{v}_2 \vec{v}_1 \cdot \vec{v}_2 \hat{n} \cdot \vec{v}_2 + \\
& \frac{28}{3} \hat{n} \times \vec{a}_2 \cdot \vec{S}_1 \vec{v}_1 \cdot \vec{v}_2 \hat{n} \cdot \vec{v}_2 + 4 \hat{n} \times \vec{S}_1 \cdot \vec{v}_2 \vec{v}_2 \cdot \vec{v}_2 \hat{n} \cdot \vec{v}_2 - 8 \hat{n} \times \vec{a}_2 \cdot \vec{S}_1 \vec{v}_2 \cdot \vec{v}_2 \hat{n} \cdot \vec{v}_2 - \frac{4}{3} \vec{a}_2 \times \vec{S}_1 \cdot \vec{v}_2 (\hat{n} \cdot \vec{v}_1)^2 - \\
& \frac{16}{3} \hat{n} \times \vec{S}_1 \cdot \vec{v}_2 \hat{n} \cdot \vec{a}_2 (\hat{n} \cdot \vec{v}_1)^2 - \frac{8}{3} \vec{S}_1 \times \vec{v}_1 \cdot \vec{v}_2 \hat{n} \cdot \vec{a}_2 \hat{n} \cdot \vec{v}_1 + \frac{4}{3} \vec{S}_1 \times \vec{v}_1 \cdot \vec{v}_2 \vec{a}_2 \cdot \vec{v}_1 + \frac{8}{3} \hat{n} \times \vec{S}_1 \cdot \vec{v}_2 \hat{n} \cdot \vec{v}_1 \vec{a}_2 \cdot \vec{v}_1 - \\
& \frac{2}{3} \vec{S}_1 \times \vec{v}_1 \cdot \vec{v}_2 \vec{a}_2 \cdot \vec{v}_2 - \frac{4}{3} \hat{n} \times \vec{S}_1 \cdot \vec{v}_2 \hat{n} \cdot \vec{v}_1 \vec{a}_2 \cdot \vec{v}_2 + \frac{2}{3} \vec{a}_2 \times \vec{S}_1 \cdot \vec{v}_2 \vec{v}_1 \cdot \vec{v}_1 + \frac{4}{3} \hat{n} \times \vec{S}_1 \cdot \vec{v}_2 \hat{n} \cdot \vec{a}_2 \vec{v}_1 \cdot \vec{v}_1 + \\
& \frac{8}{3} \vec{a}_2 \times \vec{S}_1 \cdot \vec{v}_1 \vec{v}_1 \cdot \vec{v}_2 - 2 \vec{a}_2 \times \vec{S}_1 \cdot \vec{v}_2 \vec{v}_1 \cdot \vec{v}_2 - \frac{16}{3} \hat{n} \times \vec{S}_1 \cdot \vec{v}_2 \hat{n} \cdot \vec{a}_2 \vec{v}_1 \cdot \vec{v}_2 - \frac{16}{3} \hat{n} \times \vec{a}_2 \cdot \vec{S}_1 \hat{n} \cdot \vec{v}_1 \vec{v}_1 \cdot \vec{v}_2 - \\
& \frac{4}{3} \vec{a}_2 \times \vec{S}_1 \cdot \vec{v}_1 \vec{v}_2 \cdot \vec{v}_2 + \frac{11}{3} \vec{a}_2 \times \vec{S}_1 \cdot \vec{v}_2 \vec{v}_2 \cdot \vec{v}_2 + \frac{2}{3} \hat{n} \times \vec{S}_1 \cdot \vec{v}_2 \hat{n} \cdot \vec{a}_2 \vec{v}_2 \cdot \vec{v}_2 + \frac{8}{3} \hat{n} \times \vec{a}_2 \cdot \vec{S}_1 \hat{n} \cdot \vec{v}_1 \vec{v}_2 \cdot \vec{v}_2 \Big) m_2^2 + \\
& \frac{1}{r^3} G^2 \left( -6 \hat{n} \times \vec{S}_1 \cdot \vec{v}_2 (\hat{n} \cdot \vec{v}_2)^4 + 8 \vec{S}_1 \times \vec{v}_1 \cdot \vec{v}_2 (\hat{n} \cdot \vec{v}_2)^3 + 48 \hat{n} \times \vec{S}_1 \cdot \vec{v}_2 \hat{n} \cdot \vec{v}_1 (\hat{n} \cdot \vec{v}_2)^3 - \right. \\
& 48 \hat{n} \times \vec{S}_1 \cdot \vec{v}_2 (\hat{n} \cdot \vec{v}_1)^2 (\hat{n} \cdot \vec{v}_2)^2 - 16 \vec{S}_1 \times \vec{v}_1 \cdot \vec{v}_2 \hat{n} \cdot \vec{v}_1 (\hat{n} \cdot \vec{v}_2)^2 + 8 \hat{n} \times \vec{S}_1 \cdot \vec{v}_2 \vec{v}_1 \cdot \vec{v}_1 (\hat{n} \cdot \vec{v}_2)^2 - \\
& 24 \hat{n} \times \vec{S}_1 \cdot \vec{v}_2 \vec{v}_1 \cdot \vec{v}_2 (\hat{n} \cdot \vec{v}_2)^2 + 8 \hat{n} \times \vec{S}_1 \cdot \vec{v}_2 \vec{v}_2 \cdot \vec{v}_2 (\hat{n} \cdot \vec{v}_2)^2 + 8 \vec{S}_1 \times \vec{v}_1 \cdot \vec{v}_2 \vec{v}_1 \cdot \vec{v}_2 \hat{n} \cdot \vec{v}_2 + \\
& 32 \hat{n} \times \vec{S}_1 \cdot \vec{v}_2 \hat{n} \cdot \vec{v}_1 \vec{v}_1 \cdot \vec{v}_2 \hat{n} \cdot \vec{v}_2 - 4 \vec{S}_1 \times \vec{v}_1 \cdot \vec{v}_2 \vec{v}_2 \cdot \vec{v}_2 \hat{n} \cdot \vec{v}_2 - 16 \hat{n} \times \vec{S}_1 \cdot \vec{v}_2 \hat{n} \cdot \vec{v}_1 \vec{v}_2 \cdot \vec{v}_2 \hat{n} \cdot \vec{v}_2 - \\
& 4 \hat{n} \times \vec{S}_1 \cdot \vec{v}_2 (\vec{v}_1 \cdot \vec{v}_2)^2 - 2 \hat{n} \times \vec{S}_1 \cdot \vec{v}_2 (\vec{v}_2 \cdot \vec{v}_2)^2 + 4 \hat{n} \times \vec{S}_1 \cdot \vec{v}_2 \vec{v}_1 \cdot \vec{v}_2 \vec{v}_2 \cdot \vec{v}_2 \Big) m_2^2 + \\
& G^2 \left( \frac{2}{3} \log\left(\frac{r}{R_\theta}\right) \frac{1}{\vec{a}_2 \times \vec{S}_1 \cdot \vec{v}_2} + \frac{2}{9} \frac{1}{\vec{a}_2 \times \vec{S}_1 \cdot \vec{v}_2} + \frac{2}{9} \vec{a}_2 \times \frac{1}{\vec{a}_2 \cdot \vec{S}_1} + \frac{2}{9} \vec{a}_2 \times \frac{2}{\vec{S}_1 \cdot \vec{v}_2} - \frac{2}{3} \hat{n} \times \vec{S}_1 \cdot \vec{v}_2 \hat{n} \cdot \frac{1}{\vec{a}_2} + \frac{2}{3} \hat{n} \times \vec{a}_2 \cdot \vec{S}_1 \hat{n} \cdot \frac{1}{\vec{a}_2} + \right. \\
& \frac{4}{3} \hat{n} \times \frac{1}{\vec{a}_2} \cdot \vec{S}_1 \hat{n} \cdot \vec{a}_2 - \frac{2}{3} \hat{n} \times \vec{S}_1 \cdot \vec{v}_2 \hat{n} \cdot \vec{a}_2 + 2 \hat{n} \times \vec{a}_2 \cdot \vec{S}_1 \hat{n} \cdot \vec{a}_2 + \frac{4}{3} \hat{n} \times \frac{1}{\vec{a}_2} \cdot \vec{S}_1 \hat{n} \cdot \vec{v}_2 + \frac{4}{3} \hat{n} \times \vec{a}_2 \cdot \vec{S}_1 \hat{n} \cdot \vec{v}_2 + \\
& \left. \frac{2}{3} \vec{a}_2 \times \frac{1}{\vec{a}_2} \cdot \vec{S}_1 \log\left(\frac{r}{R_\theta}\right) + \frac{2}{3} \vec{a}_2 \times \vec{S}_1 \cdot \vec{v}_2 \log\left(\frac{r}{R_\theta}\right) + \frac{-\frac{1}{3} \frac{1}{\vec{a}_2 \times \vec{S}_1 \cdot \vec{v}_2} - \frac{1}{3} \vec{a}_2 \times \frac{1}{\vec{a}_2 \cdot \vec{S}_1} - \frac{1}{3} \vec{a}_2 \times \frac{2}{\vec{S}_1 \cdot \vec{v}_2}}{\epsilon_d} \right) m_2^2 \Big\}
\end{aligned}$$

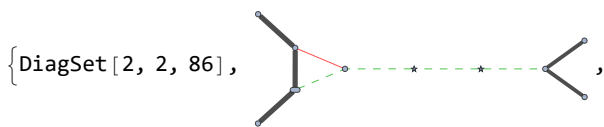

$$\begin{aligned}
& \frac{1}{r} \left( -\frac{2}{3} \hat{n} \times \vec{S}_1 \cdot \vec{a}_2 (\hat{n} \cdot \vec{v}_1)^2 + \frac{2}{3} \vec{S}_1 \times \vec{v}_2 \cdot \vec{a}_2 \hat{n} \cdot \vec{v}_1 - \frac{2}{3} \vec{S}_1 \times \vec{v}_1 \cdot \vec{a}_2 \hat{n} \cdot \vec{v}_1 + \frac{4}{3} \hat{n} \times \vec{S}_1 \cdot \vec{v}_2 \hat{n} \cdot \vec{a}_2 \hat{n} \cdot \vec{v}_1 + \right. \\
& \frac{8}{3} \hat{n} \times \vec{S}_1 \cdot \vec{a}_2 \hat{n} \cdot \vec{v}_2 \hat{n} \cdot \vec{v}_1 - \frac{2}{3} \hat{n} \times \vec{S}_1 \cdot \vec{v}_2 (\hat{n} \cdot \vec{v}_2)^2 + \frac{1}{3} \vec{S}_1 \times \vec{v}_2 \cdot \vec{a}_2 \hat{n} \cdot \vec{a}_1 + \frac{2}{3} \vec{S}_1 \times \vec{v}_1 \cdot \vec{v}_2 \hat{n} \cdot \vec{a}_2 + \frac{1}{3} \vec{S}_1 \times \vec{a}_1 \cdot \vec{v}_2 \hat{n} \cdot \vec{a}_2 + \\
& \frac{2}{3} \hat{n} \times \vec{S}_1 \cdot \vec{v}_2 \hat{n} \cdot \vec{a}_1 \hat{n} \cdot \vec{a}_2 + \frac{4}{3} \vec{S}_1 \times \vec{v}_1 \cdot \vec{a}_2 \hat{n} \cdot \vec{v}_2 + \frac{2}{3} \vec{S}_1 \times \vec{a}_1 \cdot \vec{a}_2 \hat{n} \cdot \vec{v}_2 + \frac{4}{3} \hat{n} \times \vec{S}_1 \cdot \vec{a}_2 \hat{n} \cdot \vec{a}_1 \hat{n} \cdot \vec{v}_2 - \frac{1}{3} \hat{n} \times \vec{S}_1 \cdot \vec{v}_2 \vec{a}_1 \cdot \vec{a}_2 - \\
& \frac{2}{3} \hat{n} \times \vec{S}_1 \cdot \vec{a}_2 \vec{a}_1 \cdot \vec{v}_2 - \frac{2}{3} \hat{n} \times \vec{S}_1 \cdot \vec{v}_2 \vec{v}_1 \cdot \vec{a}_2 + \frac{1}{3} \hat{n} \times \vec{S}_1 \cdot \vec{a}_2 \vec{v}_1 \cdot \vec{v}_1 - \frac{4}{3} \hat{n} \times \vec{S}_1 \cdot \vec{a}_2 \vec{v}_1 \cdot \vec{v}_2 + \frac{1}{3} \hat{n} \times \vec{S}_1 \cdot \vec{v}_2 \vec{v}_2 \cdot \vec{v}_2 \Big) m_1 m_2 G^2 + \\
& \frac{1}{r^2} \left( -\frac{2}{3} \vec{S}_1 \times \vec{v}_2 \cdot \vec{a}_2 (\hat{n} \cdot \vec{v}_1)^2 - \frac{8}{3} \hat{n} \times \vec{S}_1 \cdot \vec{v}_2 \hat{n} \cdot \vec{a}_2 (\hat{n} \cdot \vec{v}_1)^2 - \frac{16}{3} \hat{n} \times \vec{S}_1 \cdot \vec{a}_2 \hat{n} \cdot \vec{v}_2 (\hat{n} \cdot \vec{v}_1)^2 + \right. \\
& \frac{16}{3} \hat{n} \times \vec{S}_1 \cdot \vec{v}_2 (\hat{n} \cdot \vec{v}_2)^2 \hat{n} \cdot \vec{v}_1 - \frac{4}{3} \vec{S}_1 \times \vec{v}_1 \cdot \vec{v}_2 \hat{n} \cdot \vec{a}_2 \hat{n} \cdot \vec{v}_1 - \frac{8}{3} \vec{S}_1 \times \vec{v}_1 \cdot \vec{a}_2 \hat{n} \cdot \vec{v}_2 \hat{n} \cdot \vec{v}_1 + \\
& \frac{4}{3} \hat{n} \times \vec{S}_1 \cdot \vec{v}_2 \vec{v}_1 \cdot \vec{a}_2 \hat{n} \cdot \vec{v}_1 + \frac{8}{3} \hat{n} \times \vec{S}_1 \cdot \vec{a}_2 \vec{v}_1 \cdot \vec{v}_2 \hat{n} \cdot \vec{v}_1 - \frac{4}{3} \hat{n} \times \vec{S}_1 \cdot \vec{v}_2 \vec{v}_2 \cdot \vec{v}_2 \hat{n} \cdot \vec{v}_1 + \frac{4}{3} \vec{S}_1 \times \vec{v}_1 \cdot \vec{v}_2 (\hat{n} \cdot \vec{v}_2)^2 + \\
& \frac{2}{3} \vec{S}_1 \times \vec{a}_1 \cdot \vec{v}_2 (\hat{n} \cdot \vec{v}_2)^2 + \frac{8}{3} \hat{n} \times \vec{S}_1 \cdot \vec{v}_2 \hat{n} \cdot \vec{a}_1 (\hat{n} \cdot \vec{v}_2)^2 - \frac{4}{3} \hat{n} \times \vec{S}_1 \cdot \vec{v}_2 \hat{n} \cdot \vec{v}_2 \vec{a}_1 \cdot \vec{v}_2 + \frac{2}{3} \vec{S}_1 \times \vec{v}_1 \cdot \vec{v}_2 \vec{v}_1 \cdot \vec{a}_2 + \\
& \frac{1}{3} \vec{S}_1 \times \vec{v}_2 \cdot \vec{a}_2 \vec{v}_1 \cdot \vec{v}_1 + \frac{2}{3} \hat{n} \times \vec{S}_1 \cdot \vec{v}_2 \hat{n} \cdot \vec{a}_2 \vec{v}_1 \cdot \vec{v}_1 + \frac{4}{3} \hat{n} \times \vec{S}_1 \cdot \vec{a}_2 \hat{n} \cdot \vec{v}_2 \vec{v}_1 \cdot \vec{v}_1 + \frac{4}{3} \vec{S}_1 \times \vec{v}_1 \cdot \vec{a}_2 \vec{v}_1 \cdot \vec{v}_2 - \\
& \left. \frac{8}{3} \hat{n} \times \vec{S}_1 \cdot \vec{v}_2 \hat{n} \cdot \vec{v}_2 \vec{v}_1 \cdot \vec{v}_2 - \frac{2}{3} \vec{S}_1 \times \vec{v}_1 \cdot \vec{v}_2 \vec{v}_2 \cdot \vec{v}_2 - \frac{1}{3} \vec{S}_1 \times \vec{a}_1 \cdot \vec{v}_2 \vec{v}_2 \cdot \vec{v}_2 - \frac{2}{3} \hat{n} \times \vec{S}_1 \cdot \vec{v}_2 \hat{n} \cdot \vec{a}_1 \vec{v}_2 \cdot \vec{v}_2 \right) m_1 m_2 G^2 +
\end{aligned}$$

$$\begin{aligned} & \frac{1}{r^3} \left( -16 \hat{n} \times \vec{S}_1 \cdot \vec{v}_2 (\hat{n} \cdot \vec{v}_2)^2 (\hat{n} \cdot \vec{v}_1)^2 + \frac{8}{3} \hat{n} \times \vec{S}_1 \cdot \vec{v}_2 \vec{v}_2 \cdot \vec{v}_2 (\hat{n} \cdot \vec{v}_1)^2 - \frac{16}{3} \vec{S}_1 \times \vec{v}_1 \cdot \vec{v}_2 (\hat{n} \cdot \vec{v}_2)^2 \hat{n} \cdot \vec{v}_1 + \right. \\ & \quad \frac{32}{3} \hat{n} \times \vec{S}_1 \cdot \vec{v}_2 \hat{n} \cdot \vec{v}_2 \vec{v}_1 \cdot \vec{v}_2 \hat{n} \cdot \vec{v}_1 + \frac{4}{3} \vec{S}_1 \times \vec{v}_1 \cdot \vec{v}_2 \vec{v}_2 \cdot \vec{v}_2 \hat{n} \cdot \vec{v}_1 - \frac{4}{3} \hat{n} \times \vec{S}_1 \cdot \vec{v}_2 (\vec{v}_1 \cdot \vec{v}_2)^2 + \\ & \quad \left. \frac{8}{3} \hat{n} \times \vec{S}_1 \cdot \vec{v}_2 (\hat{n} \cdot \vec{v}_2)^2 \vec{v}_1 \cdot \vec{v}_1 + \frac{8}{3} \vec{S}_1 \times \vec{v}_1 \cdot \vec{v}_2 \hat{n} \cdot \vec{v}_2 \vec{v}_1 \cdot \vec{v}_2 - \frac{2}{3} \hat{n} \times \vec{S}_1 \cdot \vec{v}_2 \vec{v}_1 \cdot \vec{v}_1 \vec{v}_2 \cdot \vec{v}_2 \right) m_1 m_2 G^2 + \\ & r m_1 m_2 \left( \frac{1}{3} \log \left( \frac{r}{R_\theta} \right) \hat{n} \times \vec{S}_1 \cdot \vec{a}_2 - \frac{\hat{n} \times \vec{S}_1 \cdot \vec{a}_2}{6 \in_d} - \frac{11}{36} \hat{n} \times \vec{S}_1 \cdot \vec{a}_2 \right) G^2 + \\ & m_1 m_2 \left( -\frac{2}{3} \log \left( \frac{r}{R_\theta} \right) \vec{S}_1 \times \vec{v}_1 \cdot \vec{a}_2 + \frac{11}{18} \vec{S}_1 \times \vec{v}_1 \cdot \vec{a}_2 - \frac{11}{36} \vec{S}_1 \times \vec{v}_2 \cdot \vec{a}_2 + \frac{11}{36} \vec{S}_1 \times \vec{a}_1 \cdot \vec{a}_2 + \right. \\ & \quad \frac{1}{3} \hat{n} \times \vec{S}_1 \cdot \vec{a}_2 \hat{n} \cdot \vec{a}_1 - \frac{1}{3} \hat{n} \times \vec{S}_1 \cdot \vec{v}_2 \hat{n} \cdot \vec{a}_2 + \frac{2}{3} \hat{n} \times \vec{S}_1 \cdot \vec{a}_2 \hat{n} \cdot \vec{v}_1 - \frac{2}{3} \hat{n} \times \vec{S}_1 \cdot \vec{a}_2 \hat{n} \cdot \vec{v}_2 + \\ & \quad \left. \frac{1}{3} \vec{S}_1 \times \vec{v}_2 \cdot \vec{a}_2 \log \left( \frac{r}{R_\theta} \right) - \frac{1}{3} \vec{S}_1 \times \vec{a}_1 \cdot \vec{a}_2 \log \left( \frac{r}{R_\theta} \right) + \frac{\frac{1}{3} \vec{S}_1 \times \vec{v}_1 \cdot \vec{a}_2 - \frac{1}{6} \vec{S}_1 \times \vec{v}_2 \cdot \vec{a}_2 + \frac{1}{6} \vec{S}_1 \times \vec{a}_1 \cdot \vec{a}_2}{\in_d} \right) G^2 \Bigg\} \end{aligned}$$

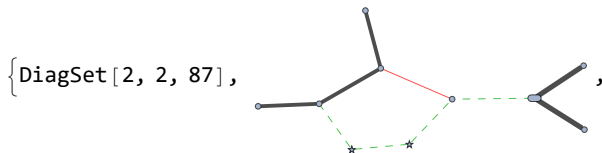

$$\begin{aligned} & -G^2 r \hat{n} \times \vec{a}_2 \cdot \vec{S}_1 m_2^2 + \frac{1}{r} G^2 \left( -\frac{5}{3} \hat{n} \times \vec{S}_1 \cdot \vec{v}_2 (\hat{n} \cdot \vec{a}_2)^2 + \frac{8}{3} \vec{S}_1 \times \vec{v}_1 \cdot \vec{v}_2 \hat{n} \cdot \vec{a}_2 - \frac{4}{3} \vec{a}_1 \times \vec{S}_1 \cdot \vec{v}_2 \hat{n} \cdot \vec{a}_2 + \vec{a}_2 \times \vec{S}_1 \cdot \vec{v}_2 \hat{n} \cdot \vec{a}_2 + \right. \\ & \quad \frac{8}{3} \hat{n} \times \vec{S}_1 \cdot \vec{v}_2 \hat{n} \cdot \vec{a}_1 \hat{n} \cdot \vec{a}_2 + \frac{16}{3} \hat{n} \times \vec{S}_1 \cdot \vec{v}_2 \hat{n} \cdot \vec{v}_1 \hat{n} \cdot \vec{a}_2 - \frac{16}{3} \hat{n} \times \vec{S}_1 \cdot \vec{v}_2 \hat{n} \cdot \vec{v}_2 \hat{n} \cdot \vec{a}_2 + \frac{4}{3} \hat{n} \times \vec{a}_2 \cdot \vec{S}_1 \hat{n} \cdot \vec{v}_2 \hat{n} \cdot \vec{a}_2 - \\ & \quad \hat{n} \times \vec{a}_2 \cdot \vec{S}_1 (\hat{n} \cdot \vec{v}_2)^2 - \hat{n} \times \vec{S}_1 \cdot \vec{v}_2 (\hat{n} \cdot \vec{v}_2)^2 + \frac{2}{3} \hat{n} \times \vec{a}_2 \cdot \vec{S}_1 (\hat{n} \cdot \vec{v}_2)^2 - \frac{2}{3} \vec{S}_1 \times \vec{v}_1 \cdot \vec{v}_2 \hat{n} \cdot \vec{a}_2 + \frac{1}{3} \vec{a}_2 \times \vec{S}_1 \cdot \vec{v}_2 \hat{n} \cdot \vec{a}_1 - \\ & \quad \frac{2}{3} \vec{a}_2 \times \vec{S}_1 \cdot \vec{v}_2 \hat{n} \cdot \vec{v}_1 + \frac{2}{3} \vec{a}_2 \times \vec{S}_1 \cdot \vec{v}_2 \hat{n} \cdot \vec{v}_1 - \frac{4}{3} \hat{n} \times \vec{S}_1 \cdot \vec{v}_2 \hat{n} \cdot \vec{a}_2 \hat{n} \cdot \vec{v}_1 - \frac{4}{3} \vec{a}_2 \times \vec{S}_1 \cdot \vec{v}_1 \hat{n} \cdot \vec{v}_2 + \frac{5}{3} \vec{a}_1 \times \vec{a}_2 \cdot \vec{S}_1 \hat{n} \cdot \vec{v}_2 + \\ & \quad \frac{10}{3} \vec{a}_2 \times \vec{S}_1 \cdot \vec{v}_1 \hat{n} \cdot \vec{v}_2 + 2 \vec{a}_2 \times \vec{S}_1 \cdot \vec{v}_2 \hat{n} \cdot \vec{v}_2 + 2 \hat{n} \times \vec{S}_1 \cdot \vec{v}_2 \hat{n} \cdot \vec{a}_2 \hat{n} \cdot \vec{v}_2 - \frac{10}{3} \hat{n} \times \vec{a}_2 \cdot \vec{S}_1 \hat{n} \cdot \vec{a}_1 \hat{n} \cdot \vec{v}_2 + \\ & \quad \frac{8}{3} \hat{n} \times \vec{a}_2 \cdot \vec{S}_1 \hat{n} \cdot \vec{v}_1 \hat{n} \cdot \vec{v}_2 - \frac{20}{3} \hat{n} \times \vec{a}_2 \cdot \vec{S}_1 \hat{n} \cdot \vec{v}_1 \hat{n} \cdot \vec{v}_2 + \frac{2}{3} \hat{n} \times \vec{S}_1 \cdot \vec{v}_2 \vec{a}_2 \cdot \vec{v}_1 - \hat{n} \times \vec{S}_1 \cdot \vec{v}_2 \vec{a}_2 \cdot \vec{v}_2 - \\ & \quad \frac{4}{3} \hat{n} \times \vec{S}_1 \cdot \vec{v}_2 \vec{a}_1 \cdot \vec{a}_2 + \frac{5}{3} \hat{n} \times \vec{a}_2 \cdot \vec{S}_1 \vec{a}_1 \cdot \vec{v}_2 + \frac{1}{3} \hat{n} \times \vec{S}_1 \cdot \vec{v}_2 \vec{a}_2 \cdot \vec{a}_2 - \frac{8}{3} \hat{n} \times \vec{S}_1 \cdot \vec{v}_2 \vec{a}_2 \cdot \vec{v}_1 + \frac{5}{3} \hat{n} \times \vec{S}_1 \cdot \vec{v}_2 \vec{a}_2 \cdot \vec{v}_2 + \\ & \quad \left. \frac{1}{3} \hat{n} \times \vec{a}_2 \cdot \vec{S}_1 \vec{a}_2 \cdot \vec{v}_2 - \frac{4}{3} \hat{n} \times \vec{a}_2 \cdot \vec{S}_1 \vec{v}_1 \cdot \vec{v}_2 + \frac{10}{3} \hat{n} \times \vec{a}_2 \cdot \vec{S}_1 \vec{v}_1 \cdot \vec{v}_2 + \hat{n} \times \vec{S}_1 \cdot \vec{v}_2 \vec{v}_2 \cdot \vec{v}_2 + \frac{5}{3} \hat{n} \times \vec{a}_2 \cdot \vec{S}_1 \vec{v}_2 \cdot \vec{v}_2 \right) m_2^2 + \\ & \frac{1}{r^2} G^2 \left( -2 \hat{n} \times \vec{S}_1 \cdot \vec{v}_2 (\hat{n} \cdot \vec{v}_2)^3 - \frac{8}{3} \hat{n} \times \vec{a}_2 \cdot \vec{S}_1 (\hat{n} \cdot \vec{v}_2)^3 + 2 \vec{S}_1 \times \vec{v}_1 \cdot \vec{v}_2 (\hat{n} \cdot \vec{v}_2)^2 - \vec{a}_1 \times \vec{S}_1 \cdot \vec{v}_2 (\hat{n} \cdot \vec{v}_2)^2 + \right. \\ & \quad \frac{2}{3} \vec{a}_2 \times \vec{S}_1 \cdot \vec{v}_1 (\hat{n} \cdot \vec{v}_2)^2 + \frac{31}{6} \vec{a}_2 \times \vec{S}_1 \cdot \vec{v}_2 (\hat{n} \cdot \vec{v}_2)^2 + 4 \hat{n} \times \vec{S}_1 \cdot \vec{v}_2 \hat{n} \cdot \vec{a}_1 (\hat{n} \cdot \vec{v}_2)^2 - \frac{38}{3} \hat{n} \times \vec{S}_1 \cdot \vec{v}_2 \hat{n} \cdot \vec{a}_2 (\hat{n} \cdot \vec{v}_2)^2 + \\ & \quad 8 \hat{n} \times \vec{S}_1 \cdot \vec{v}_2 \hat{n} \cdot \vec{v}_1 (\hat{n} \cdot \vec{v}_2)^2 - \frac{8}{3} \hat{n} \times \vec{a}_2 \cdot \vec{S}_1 \hat{n} \cdot \vec{v}_1 (\hat{n} \cdot \vec{v}_2)^2 + \frac{40}{3} \hat{n} \times \vec{a}_2 \cdot \vec{S}_1 (\hat{n} \cdot \vec{v}_1)^2 \hat{n} \cdot \vec{v}_2 + \\ & \quad \frac{16}{3} \vec{S}_1 \times \vec{v}_1 \cdot \vec{v}_2 \hat{n} \cdot \vec{a}_2 \hat{n} \cdot \vec{v}_2 - \frac{20}{3} \vec{a}_2 \times \vec{S}_1 \cdot \vec{v}_1 \hat{n} \cdot \vec{v}_1 \hat{n} \cdot \vec{v}_2 - 4 \vec{a}_2 \times \vec{S}_1 \cdot \vec{v}_2 \hat{n} \cdot \vec{v}_1 \hat{n} \cdot \vec{v}_2 + \frac{64}{3} \hat{n} \times \vec{S}_1 \cdot \vec{v}_2 \hat{n} \cdot \vec{a}_2 \hat{n} \cdot \vec{v}_1 \hat{n} \cdot \vec{v}_2 - \\ & \quad 2 \hat{n} \times \vec{S}_1 \cdot \vec{v}_2 \vec{a}_1 \cdot \vec{v}_2 \hat{n} \cdot \vec{v}_2 - \frac{16}{3} \hat{n} \times \vec{S}_1 \cdot \vec{v}_2 \vec{a}_2 \cdot \vec{v}_1 \hat{n} \cdot \vec{v}_2 + \frac{13}{3} \hat{n} \times \vec{S}_1 \cdot \vec{v}_2 \vec{a}_2 \cdot \vec{v}_2 \hat{n} \cdot \vec{v}_2 - \frac{10}{3} \hat{n} \times \vec{a}_2 \cdot \vec{S}_1 \vec{v}_1 \cdot \vec{v}_1 \hat{n} \cdot \vec{v}_2 - \\ & \quad \left. 4 \hat{n} \times \vec{S}_1 \cdot \vec{v}_2 \vec{v}_1 \cdot \vec{v}_2 \hat{n} \cdot \vec{v}_2 + \frac{4}{3} \hat{n} \times \vec{a}_2 \cdot \vec{S}_1 \vec{v}_1 \cdot \vec{v}_2 \hat{n} \cdot \vec{v}_2 + 2 \hat{n} \times \vec{S}_1 \cdot \vec{v}_2 \vec{v}_2 \cdot \vec{v}_2 \hat{n} \cdot \vec{v}_2 - \frac{2}{3} \vec{a}_2 \times \vec{S}_1 \cdot \vec{v}_2 (\hat{n} \cdot \vec{v}_1)^2 - \right. \end{aligned}$$

$$\begin{aligned}
& \frac{32}{3} \hat{n} \times \vec{S}_1 \cdot \vec{v}_2 \hat{n} \cdot \vec{a}_2 (\hat{n} \cdot \vec{v}_1)^2 - \frac{16}{3} \vec{S}_1 \times \vec{v}_1 \cdot \vec{v}_2 \hat{n} \cdot \vec{a}_2 \hat{n} \cdot \vec{v}_1 + \frac{8}{3} \vec{S}_1 \times \vec{v}_1 \cdot \vec{v}_2 \vec{a}_2 \cdot \vec{v}_1 + \frac{16}{3} \hat{n} \times \vec{S}_1 \cdot \vec{v}_2 \hat{n} \cdot \vec{v}_1 \vec{a}_2 \cdot \vec{v}_1 - \\
& \frac{5}{3} \vec{S}_1 \times \vec{v}_1 \cdot \vec{v}_2 \vec{a}_2 \cdot \vec{v}_2 - \frac{10}{3} \hat{n} \times \vec{S}_1 \cdot \vec{v}_2 \hat{n} \cdot \vec{v}_1 \vec{a}_2 \cdot \vec{v}_2 + \frac{1}{3} \vec{a}_2 \times \vec{S}_1 \cdot \vec{v}_2 \vec{v}_1 \cdot \vec{v}_1 + \frac{8}{3} \hat{n} \times \vec{S}_1 \cdot \vec{v}_2 \hat{n} \cdot \vec{a}_2 \vec{v}_1 \cdot \vec{v}_1 + \\
& \frac{10}{3} \vec{a}_2 \times \vec{S}_1 \cdot \vec{v}_1 \vec{v}_1 \cdot \vec{v}_2 + 2 \vec{a}_2 \times \vec{S}_1 \cdot \vec{v}_2 \vec{v}_1 \cdot \vec{v}_2 - \frac{16}{3} \hat{n} \times \vec{S}_1 \cdot \vec{v}_2 \hat{n} \cdot \vec{a}_2 \vec{v}_1 \cdot \vec{v}_2 - \frac{20}{3} \hat{n} \times \vec{a}_2 \cdot \vec{S}_1 \hat{n} \cdot \vec{v}_1 \vec{v}_1 \cdot \vec{v}_2 - \\
& 2 \vec{S}_1 \times \vec{v}_1 \cdot \vec{v}_2 \vec{v}_2 \cdot \vec{v}_2 + \vec{a}_1 \times \vec{S}_1 \cdot \vec{v}_2 \vec{v}_2 \cdot \vec{v}_2 + \frac{5}{3} \vec{a}_2 \times \vec{S}_1 \cdot \vec{v}_1 \vec{v}_2 \cdot \vec{v}_2 + \frac{1}{6} \vec{a}_2 \times \vec{S}_1 \cdot \vec{v}_2 \vec{v}_2 \cdot \vec{v}_2 - 2 \hat{n} \times \vec{S}_1 \cdot \vec{v}_2 \hat{n} \cdot \vec{a}_1 \vec{v}_2 \cdot \vec{v}_2 - \\
& \frac{1}{3} \hat{n} \times \vec{S}_1 \cdot \vec{v}_2 \hat{n} \cdot \vec{a}_2 \vec{v}_2 \cdot \vec{v}_2 - 4 \hat{n} \times \vec{S}_1 \cdot \vec{v}_2 \hat{n} \cdot \vec{v}_1 \vec{v}_2 \cdot \vec{v}_2 - \frac{10}{3} \hat{n} \times \vec{a}_2 \cdot \vec{S}_1 \hat{n} \cdot \vec{v}_1 \vec{v}_2 \cdot \vec{v}_2 \Big) m_2^2 + \frac{1}{r^3} \\
& G^2 \left( -3 \hat{n} \times \vec{S}_1 \cdot \vec{v}_2 (\hat{n} \cdot \vec{v}_2)^4 + 2 \vec{S}_1 \times \vec{v}_1 \cdot \vec{v}_2 (\hat{n} \cdot \vec{v}_2)^3 + 12 \hat{n} \times \vec{S}_1 \cdot \vec{v}_2 \hat{n} \cdot \vec{v}_1 (\hat{n} \cdot \vec{v}_2)^3 - 24 \hat{n} \times \vec{S}_1 \cdot \vec{v}_2 (\hat{n} \cdot \vec{v}_1)^2 (\hat{n} \cdot \vec{v}_2)^2 - \right. \\
& 8 \vec{S}_1 \times \vec{v}_1 \cdot \vec{v}_2 \hat{n} \cdot \vec{v}_1 (\hat{n} \cdot \vec{v}_2)^2 + 4 \hat{n} \times \vec{S}_1 \cdot \vec{v}_2 \vec{v}_1 \cdot \vec{v}_1 (\hat{n} \cdot \vec{v}_2)^2 - 6 \hat{n} \times \vec{S}_1 \cdot \vec{v}_2 \vec{v}_1 \cdot \vec{v}_2 (\hat{n} \cdot \vec{v}_2)^2 + \\
& 4 \hat{n} \times \vec{S}_1 \cdot \vec{v}_2 \vec{v}_2 \cdot \vec{v}_2 (\hat{n} \cdot \vec{v}_2)^2 + 4 \vec{S}_1 \times \vec{v}_1 \cdot \vec{v}_2 \vec{v}_1 \cdot \vec{v}_2 \hat{n} \cdot \vec{v}_2 + 16 \hat{n} \times \vec{S}_1 \cdot \vec{v}_2 \hat{n} \cdot \vec{v}_1 \vec{v}_1 \cdot \vec{v}_2 \hat{n} \cdot \vec{v}_2 - \\
& 2 \vec{S}_1 \times \vec{v}_1 \cdot \vec{v}_2 \vec{v}_2 \cdot \vec{v}_2 \hat{n} \cdot \vec{v}_2 - 8 \hat{n} \times \vec{S}_1 \cdot \vec{v}_2 \hat{n} \cdot \vec{v}_1 \vec{v}_2 \cdot \vec{v}_2 \hat{n} \cdot \vec{v}_2 - 2 \hat{n} \times \vec{S}_1 \cdot \vec{v}_2 (\vec{v}_1 \cdot \vec{v}_2)^2 - \hat{n} \times \vec{S}_1 \cdot \vec{v}_2 (\vec{v}_2 \cdot \vec{v}_2)^2 + \\
& 8 \hat{n} \times \vec{S}_1 \cdot \vec{v}_2 (\hat{n} \cdot \vec{v}_1)^2 \vec{v}_2 \cdot \vec{v}_2 + 4 \vec{S}_1 \times \vec{v}_1 \cdot \vec{v}_2 \hat{n} \cdot \vec{v}_1 \vec{v}_2 \cdot \vec{v}_2 - 2 \hat{n} \times \vec{S}_1 \cdot \vec{v}_2 \vec{v}_1 \cdot \vec{v}_1 \vec{v}_2 \cdot \vec{v}_2 + 2 \hat{n} \times \vec{S}_1 \cdot \vec{v}_2 \vec{v}_1 \cdot \vec{v}_2 \vec{v}_2 \cdot \vec{v}_2 \Big) m_2^2 + \\
& G^2 \left( -2 \frac{1}{\vec{a}_2 \times \vec{S}_1 \cdot \vec{v}_1} + \frac{4}{9} \frac{1}{\vec{a}_2 \times \vec{S}_1 \cdot \vec{v}_2} - \frac{1}{\vec{a}_1 \times \vec{a}_2 \cdot \vec{S}_1} + \frac{2}{9} \frac{1}{\vec{a}_2 \times \vec{a}_2 \cdot \vec{S}_1} + \frac{7}{9} \frac{1}{\vec{a}_2 \times \vec{S}_1 \cdot \vec{v}_2} + \frac{2}{3} \hat{n} \times \vec{S}_1 \cdot \vec{v}_2 \hat{n} \cdot \frac{1}{\vec{a}_2} - \frac{1}{3} \hat{n} \times \vec{a}_2 \cdot \vec{S}_1 \hat{n} \cdot \frac{1}{\vec{a}_2} - \right. \\
& \frac{2}{3} \hat{n} \times \vec{a}_2 \cdot \vec{S}_1 \hat{n} \cdot \vec{a}_2 - \frac{4}{3} \hat{n} \times \vec{S}_1 \cdot \vec{v}_2 \hat{n} \cdot \vec{a}_2 - \frac{4}{3} \hat{n} \times \vec{a}_2 \cdot \vec{S}_1 \hat{n} \cdot \vec{v}_2 + \frac{5}{3} \hat{n} \times \vec{a}_2 \cdot \vec{S}_1 \hat{n} \cdot \vec{v}_2 - \frac{2}{3} \frac{1}{\vec{a}_2 \times \vec{S}_1 \cdot \vec{v}_2} \log \left( \frac{r}{R_0} \right) - \\
& \left. \frac{1}{3} \frac{1}{\vec{a}_2 \times \vec{a}_2 \cdot \vec{S}_1} \log \left( \frac{r}{R_0} \right) + \frac{1}{3} \frac{1}{\vec{a}_2 \times \vec{S}_1 \cdot \vec{v}_2} \log \left( \frac{r}{R_0} \right) + \frac{\frac{1}{3} \frac{1}{\vec{a}_2 \times \vec{S}_1 \cdot \vec{v}_2} + \frac{1}{6} \frac{1}{\vec{a}_2 \times \vec{a}_2 \cdot \vec{S}_1} - \frac{1}{6} \frac{1}{\vec{a}_2 \times \vec{S}_1 \cdot \vec{v}_2}}{\epsilon_d} \right) m_2^2 \Big\}
\end{aligned}$$

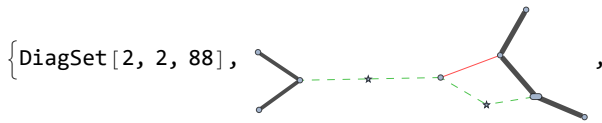

$$\begin{aligned}
& \frac{1}{r} \left( -\frac{5}{2} \hat{n} \times \vec{S}_1 \cdot \vec{a}_2 (\hat{n} \cdot \vec{v}_1)^2 - 2 \hat{n} \times \vec{S}_1 \cdot \vec{a}_2 (\hat{n} \cdot \vec{v}_1)^2 - \frac{8}{3} \vec{S}_1 \times \vec{v}_1 \cdot \vec{a}_2 \hat{n} \cdot \vec{v}_1 + 3 \vec{S}_1 \times \vec{v}_2 \cdot \vec{a}_2 \hat{n} \cdot \vec{v}_1 - \vec{S}_1 \times \vec{a}_1 \cdot \vec{a}_2 \hat{n} \cdot \vec{v}_1 - \right. \\
& \frac{7}{3} \vec{S}_1 \times \vec{v}_1 \cdot \vec{a}_2 \hat{n} \cdot \vec{v}_1 - \frac{1}{3} \hat{n} \times \vec{S}_1 \cdot \vec{v}_1 \hat{n} \cdot \vec{a}_2 \hat{n} \cdot \vec{v}_1 - \hat{n} \times \vec{S}_1 \cdot \vec{a}_2 \hat{n} \cdot \vec{a}_1 \hat{n} \cdot \vec{v}_1 + \frac{1}{3} \hat{n} \times \vec{S}_1 \cdot \vec{v}_1 \hat{n} \cdot \vec{a}_2 \hat{n} \cdot \vec{v}_1 + \\
& 6 \hat{n} \times \vec{S}_1 \cdot \vec{v}_2 \hat{n} \cdot \vec{a}_2 \hat{n} \cdot \vec{v}_1 + 12 \hat{n} \times \vec{S}_1 \cdot \vec{a}_2 \hat{n} \cdot \vec{v}_2 \hat{n} \cdot \vec{v}_1 + 2 \hat{n} \times \vec{S}_1 \cdot \vec{v}_2 \hat{n} \cdot \vec{v}_2 \hat{n} \cdot \vec{v}_1 - \frac{1}{3} \hat{n} \times \vec{S}_1 \cdot \vec{a}_1 (\hat{n} \cdot \vec{v}_2)^2 - \\
& \frac{1}{3} \hat{n} \times \vec{S}_1 \cdot \vec{v}_1 (\hat{n} \cdot \vec{v}_2)^2 - 4 \hat{n} \times \vec{S}_1 \cdot \vec{v}_2 (\hat{n} \cdot \vec{v}_2)^2 - \vec{S}_1 \times \vec{v}_1 \cdot \vec{a}_2 \hat{n} \cdot \vec{a}_1 + \vec{S}_1 \times \vec{v}_2 \cdot \vec{a}_2 \hat{n} \cdot \vec{a}_1 + 3 \vec{S}_1 \times \vec{v}_1 \cdot \vec{v}_2 \hat{n} \cdot \vec{a}_2 + \\
& \vec{S}_1 \times \vec{a}_1 \cdot \vec{v}_2 \hat{n} \cdot \vec{a}_2 + 2 \hat{n} \times \vec{S}_1 \cdot \vec{v}_2 \hat{n} \cdot \vec{a}_1 \hat{n} \cdot \vec{a}_2 + \frac{5}{6} \vec{S}_1 \times \vec{a}_1 \cdot \vec{v}_2 \hat{n} \cdot \vec{v}_2 + \frac{13}{2} \vec{S}_1 \times \vec{v}_1 \cdot \vec{a}_2 \hat{n} \cdot \vec{v}_2 + \frac{5}{6} \vec{S}_1 \times \vec{v}_1 \cdot \vec{v}_2 \hat{n} \cdot \vec{v}_2 + \\
& \frac{5}{2} \vec{S}_1 \times \vec{a}_1 \cdot \vec{a}_2 \hat{n} \cdot \vec{v}_2 + 2 \hat{n} \times \vec{S}_1 \cdot \vec{v}_2 \hat{n} \cdot \vec{a}_1 \hat{n} \cdot \vec{v}_2 + 4 \hat{n} \times \vec{S}_1 \cdot \vec{a}_2 \hat{n} \cdot \vec{a}_1 \hat{n} \cdot \vec{v}_2 + \hat{n} \times \vec{S}_1 \cdot \vec{v}_1 \hat{n} \cdot \vec{a}_2 \hat{n} \cdot \vec{v}_2 + \\
& \hat{n} \times \vec{S}_1 \cdot \vec{a}_1 \hat{n} \cdot \vec{a}_2 \hat{n} \cdot \vec{v}_2 + \frac{1}{2} \hat{n} \times \vec{S}_1 \cdot \vec{v}_1 \vec{a}_1 \cdot \vec{a}_2 - \hat{n} \times \vec{S}_1 \cdot \vec{v}_2 \vec{a}_1 \cdot \vec{a}_2 - \hat{n} \times \vec{S}_1 \cdot \vec{v}_2 \vec{a}_1 \cdot \vec{v}_2 - 2 \hat{n} \times \vec{S}_1 \cdot \vec{a}_2 \vec{a}_1 \cdot \vec{v}_2 + \\
& \frac{1}{6} \hat{n} \times \vec{S}_1 \cdot \vec{v}_1 \vec{v}_1 \cdot \vec{a}_2 + \hat{n} \times \vec{S}_1 \cdot \vec{a}_2 \vec{v}_1 \cdot \vec{a}_1 + \frac{1}{3} \hat{n} \times \vec{S}_1 \cdot \vec{v}_1 \vec{v}_1 \cdot \vec{a}_2 - 3 \hat{n} \times \vec{S}_1 \cdot \vec{v}_2 \vec{v}_1 \cdot \vec{a}_2 + \frac{1}{2} \hat{n} \times \vec{S}_1 \cdot \vec{a}_1 \vec{v}_1 \cdot \vec{a}_2 + \\
& \frac{3}{2} \hat{n} \times \vec{S}_1 \cdot \vec{a}_2 \vec{v}_1 \cdot \vec{v}_1 + \hat{n} \times \vec{S}_1 \cdot \vec{a}_2 \vec{v}_1 \cdot \vec{v}_1 - 6 \hat{n} \times \vec{S}_1 \cdot \vec{a}_2 \vec{v}_1 \cdot \vec{v}_2 - \hat{n} \times \vec{S}_1 \cdot \vec{v}_2 \vec{v}_1 \cdot \vec{v}_2 - \frac{1}{2} \hat{n} \times \vec{S}_1 \cdot \vec{v}_1 \vec{v}_2 \cdot \vec{a}_2 - \\
& \frac{1}{2} \hat{n} \times \vec{S}_1 \cdot \vec{a}_1 \vec{v}_2 \cdot \vec{a}_2 + \frac{1}{6} \hat{n} \times \vec{S}_1 \cdot \vec{a}_1 \vec{v}_2 \cdot \vec{v}_2 + \frac{1}{6} \hat{n} \times \vec{S}_1 \cdot \vec{v}_1 \vec{v}_2 \cdot \vec{v}_2 + 2 \hat{n} \times \vec{S}_1 \cdot \vec{v}_2 \vec{v}_2 \cdot \vec{v}_2 \Big) m_1 m_2 G^2 + \frac{1}{r^2} \\
& \left( 2 \hat{n} \times \vec{S}_1 \cdot \vec{a}_2 (\hat{n} \cdot \vec{v}_1)^3 + \frac{5}{2} \vec{S}_1 \times \vec{v}_1 \cdot \vec{a}_2 (\hat{n} \cdot \vec{v}_1)^2 - 2 \vec{S}_1 \times \vec{v}_2 \cdot \vec{a}_2 (\hat{n} \cdot \vec{v}_1)^2 - 8 \hat{n} \times \vec{S}_1 \cdot \vec{v}_2 \hat{n} \cdot \vec{a}_2 (\hat{n} \cdot \vec{v}_1)^2 - \right.
\end{aligned}$$

$$\begin{aligned}
& 10 \hat{n} \times \vec{S}_1 \cdot \vec{v}_2 \hat{n} \cdot \vec{v}_2 (\hat{n} \cdot \vec{v}_1)^2 - 16 \hat{n} \times \vec{S}_1 \cdot \vec{a}_2 \hat{n} \cdot \vec{v}_2 (\hat{n} \cdot \vec{v}_1)^2 + \frac{4}{3} \hat{n} \times \vec{S}_1 \cdot \vec{v}_1 (\hat{n} \cdot \vec{v}_2)^2 \hat{n} \cdot \vec{v}_1 + \\
& 24 \hat{n} \times \vec{S}_1 \cdot \vec{v}_2 (\hat{n} \cdot \vec{v}_2)^2 \hat{n} \cdot \vec{v}_1 - 4 \vec{S}_1 \times \vec{v}_1 \cdot \vec{v}_2 \hat{n} \cdot \vec{a}_2 \hat{n} \cdot \vec{v}_1 - \frac{17}{3} \vec{S}_1 \times \vec{v}_1 \cdot \vec{v}_2 \hat{n} \cdot \vec{v}_2 \hat{n} \cdot \vec{v}_1 - 2 \vec{S}_1 \times \vec{a}_1 \cdot \vec{v}_2 \hat{n} \cdot \vec{v}_2 \hat{n} \cdot \vec{v}_1 - \\
& 9 \vec{S}_1 \times \vec{v}_1 \cdot \vec{a}_2 \hat{n} \cdot \vec{v}_2 \hat{n} \cdot \vec{v}_1 - 4 \hat{n} \times \vec{S}_1 \cdot \vec{v}_2 \hat{n} \cdot \vec{a}_1 \hat{n} \cdot \vec{v}_2 \hat{n} \cdot \vec{v}_1 - 4 \hat{n} \times \vec{S}_1 \cdot \vec{v}_1 \hat{n} \cdot \vec{a}_2 \hat{n} \cdot \vec{v}_2 \hat{n} \cdot \vec{v}_1 + \\
& \hat{n} \times \vec{S}_1 \cdot \vec{v}_2 \vec{a}_1 \cdot \vec{v}_2 \hat{n} \cdot \vec{v}_1 - \hat{n} \times \vec{S}_1 \cdot \vec{v}_1 \vec{v}_1 \cdot \vec{a}_2 \hat{n} \cdot \vec{v}_1 + 4 \hat{n} \times \vec{S}_1 \cdot \vec{v}_2 \vec{v}_1 \cdot \vec{a}_2 \hat{n} \cdot \vec{v}_1 - 2 \hat{n} \times \vec{S}_1 \cdot \vec{a}_2 \vec{v}_1 \cdot \vec{v}_1 \hat{n} \cdot \vec{v}_1 + \\
& 5 \hat{n} \times \vec{S}_1 \cdot \vec{v}_2 \vec{v}_1 \cdot \vec{v}_2 \hat{n} \cdot \vec{v}_1 + 8 \hat{n} \times \vec{S}_1 \cdot \vec{a}_2 \vec{v}_1 \cdot \vec{v}_2 \hat{n} \cdot \vec{v}_1 + \hat{n} \times \vec{S}_1 \cdot \vec{v}_1 \vec{v}_2 \cdot \vec{a}_2 \hat{n} \cdot \vec{v}_1 - \frac{1}{3} \hat{n} \times \vec{S}_1 \cdot \vec{v}_1 \vec{v}_2 \cdot \vec{v}_2 \hat{n} \cdot \vec{v}_1 - \\
& 6 \hat{n} \times \vec{S}_1 \cdot \vec{v}_2 \vec{v}_2 \cdot \vec{v}_2 \hat{n} \cdot \vec{v}_1 + \frac{4}{3} \hat{n} \times \vec{S}_1 \cdot \vec{v}_1 (\hat{n} \cdot \vec{v}_2)^3 + \frac{4}{3} \hat{n} \times \vec{S}_1 \cdot \vec{a}_1 (\hat{n} \cdot \vec{v}_2)^3 + 6 \vec{S}_1 \times \vec{v}_1 \cdot \vec{v}_2 (\hat{n} \cdot \vec{v}_2)^2 + \\
& 2 \vec{S}_1 \times \vec{a}_1 \cdot \vec{v}_2 (\hat{n} \cdot \vec{v}_2)^2 + 8 \hat{n} \times \vec{S}_1 \cdot \vec{v}_2 \hat{n} \cdot \vec{a}_1 (\hat{n} \cdot \vec{v}_2)^2 - 2 \vec{S}_1 \times \vec{v}_1 \cdot \vec{v}_2 \hat{n} \cdot \vec{a}_1 \hat{n} \cdot \vec{v}_2 + \frac{1}{2} \vec{S}_1 \times \vec{v}_1 \cdot \vec{v}_2 \vec{a}_1 \cdot \vec{v}_2 + \\
& \hat{n} \times \vec{S}_1 \cdot \vec{v}_1 \hat{n} \cdot \vec{v}_2 \vec{a}_1 \cdot \vec{v}_2 - 4 \hat{n} \times \vec{S}_1 \cdot \vec{v}_2 \hat{n} \cdot \vec{v}_2 \vec{a}_1 \cdot \vec{v}_2 + 2 \hat{n} \times \vec{S}_1 \cdot \vec{v}_2 \hat{n} \cdot \vec{v}_2 \vec{v}_1 \cdot \vec{a}_1 + 2 \vec{S}_1 \times \vec{v}_1 \cdot \vec{v}_2 \vec{v}_1 \cdot \vec{a}_2 + \\
& \hat{n} \times \vec{S}_1 \cdot \vec{v}_1 \hat{n} \cdot \vec{v}_2 \vec{v}_1 \cdot \vec{a}_2 - \frac{3}{2} \vec{S}_1 \times \vec{v}_1 \cdot \vec{a}_2 \vec{v}_1 \cdot \vec{v}_1 + \vec{S}_1 \times \vec{v}_2 \cdot \vec{a}_2 \vec{v}_1 \cdot \vec{v}_1 + 2 \hat{n} \times \vec{S}_1 \cdot \vec{v}_2 \hat{n} \cdot \vec{a}_2 \vec{v}_1 \cdot \vec{v}_1 + \\
& 3 \hat{n} \times \vec{S}_1 \cdot \vec{v}_2 \hat{n} \cdot \vec{v}_2 \vec{v}_1 \cdot \vec{v}_1 + 4 \hat{n} \times \vec{S}_1 \cdot \vec{a}_2 \hat{n} \cdot \vec{v}_2 \vec{v}_1 \cdot \vec{v}_1 + \frac{7}{3} \vec{S}_1 \times \vec{v}_1 \cdot \vec{v}_2 \vec{v}_1 \cdot \vec{v}_2 + \frac{1}{2} \vec{S}_1 \times \vec{a}_1 \cdot \vec{v}_2 \vec{v}_1 \cdot \vec{v}_2 + \\
& \frac{9}{2} \vec{S}_1 \times \vec{v}_1 \cdot \vec{a}_2 \vec{v}_1 \cdot \vec{v}_2 + \hat{n} \times \vec{S}_1 \cdot \vec{v}_2 \hat{n} \cdot \vec{a}_1 \vec{v}_1 \cdot \vec{v}_2 + \hat{n} \times \vec{S}_1 \cdot \vec{v}_1 \hat{n} \cdot \vec{a}_2 \vec{v}_1 \cdot \vec{v}_2 + \frac{1}{3} \hat{n} \times \vec{S}_1 \cdot \vec{v}_1 \hat{n} \cdot \vec{v}_2 \vec{v}_1 \cdot \vec{v}_2 - \\
& 12 \hat{n} \times \vec{S}_1 \cdot \vec{v}_2 \hat{n} \cdot \vec{v}_2 \vec{v}_1 \cdot \vec{v}_2 + \hat{n} \times \vec{S}_1 \cdot \vec{a}_1 \hat{n} \cdot \vec{v}_2 \vec{v}_1 \cdot \vec{v}_2 - 3 \vec{S}_1 \times \vec{v}_1 \cdot \vec{v}_2 \vec{v}_2 \cdot \vec{v}_2 - \vec{S}_1 \times \vec{a}_1 \cdot \vec{v}_2 \vec{v}_2 \cdot \vec{v}_2 - \\
& 2 \hat{n} \times \vec{S}_1 \cdot \vec{v}_2 \hat{n} \cdot \vec{a}_1 \vec{v}_2 \cdot \vec{v}_2 - \hat{n} \times \vec{S}_1 \cdot \vec{v}_1 \hat{n} \cdot \vec{v}_2 \vec{v}_2 \cdot \vec{v}_2 - \hat{n} \times \vec{S}_1 \cdot \vec{a}_1 \hat{n} \cdot \vec{v}_2 \vec{v}_2 \cdot \vec{v}_2 \Big) m_1 m_2 G^2 + \frac{1}{r^3} \\
& \left( 12 \hat{n} \times \vec{S}_1 \cdot \vec{v}_2 \hat{n} \cdot \vec{v}_2 (\hat{n} \cdot \vec{v}_1)^3 - 48 \hat{n} \times \vec{S}_1 \cdot \vec{v}_2 (\hat{n} \cdot \vec{v}_2)^2 (\hat{n} \cdot \vec{v}_1)^2 + 10 \vec{S}_1 \times \vec{v}_1 \cdot \vec{v}_2 \hat{n} \cdot \vec{v}_2 (\hat{n} \cdot \vec{v}_1)^2 - \right. \\
& 6 \hat{n} \times \vec{S}_1 \cdot \vec{v}_2 \vec{v}_1 \cdot \vec{v}_2 (\hat{n} \cdot \vec{v}_1)^2 + 8 \hat{n} \times \vec{S}_1 \cdot \vec{v}_2 \vec{v}_2 \cdot \vec{v}_2 (\hat{n} \cdot \vec{v}_1)^2 - 8 \hat{n} \times \vec{S}_1 \cdot \vec{v}_1 (\hat{n} \cdot \vec{v}_2)^3 \hat{n} \cdot \vec{v}_1 - \\
& 16 \vec{S}_1 \times \vec{v}_1 \cdot \vec{v}_2 (\hat{n} \cdot \vec{v}_2)^2 \hat{n} \cdot \vec{v}_1 - 8 \hat{n} \times \vec{S}_1 \cdot \vec{v}_2 \hat{n} \cdot \vec{v}_2 \vec{v}_1 \cdot \vec{v}_1 \hat{n} \cdot \vec{v}_1 - 4 \vec{S}_1 \times \vec{v}_1 \cdot \vec{v}_2 \vec{v}_1 \cdot \vec{v}_2 \hat{n} \cdot \vec{v}_1 - \\
& 4 \hat{n} \times \vec{S}_1 \cdot \vec{v}_1 \hat{n} \cdot \vec{v}_2 \vec{v}_1 \cdot \vec{v}_2 \hat{n} \cdot \vec{v}_1 + 32 \hat{n} \times \vec{S}_1 \cdot \vec{v}_2 \hat{n} \cdot \vec{v}_2 \vec{v}_1 \cdot \vec{v}_2 \hat{n} \cdot \vec{v}_1 + 4 \vec{S}_1 \times \vec{v}_1 \cdot \vec{v}_2 \vec{v}_2 \cdot \vec{v}_2 \hat{n} \cdot \vec{v}_1 + \\
& 4 \hat{n} \times \vec{S}_1 \cdot \vec{v}_1 \hat{n} \cdot \vec{v}_2 \vec{v}_2 \cdot \vec{v}_2 \hat{n} \cdot \vec{v}_1 + \hat{n} \times \vec{S}_1 \cdot \vec{v}_1 (\vec{v}_1 \cdot \vec{v}_2)^2 - 4 \hat{n} \times \vec{S}_1 \cdot \vec{v}_2 (\vec{v}_1 \cdot \vec{v}_2)^2 + 8 \hat{n} \times \vec{S}_1 \cdot \vec{v}_2 (\hat{n} \cdot \vec{v}_2)^2 \vec{v}_1 \cdot \vec{v}_1 - \\
& 3 \vec{S}_1 \times \vec{v}_1 \cdot \vec{v}_2 \hat{n} \cdot \vec{v}_2 \vec{v}_1 \cdot \vec{v}_1 + 4 \hat{n} \times \vec{S}_1 \cdot \vec{v}_1 (\hat{n} \cdot \vec{v}_2)^2 \vec{v}_1 \cdot \vec{v}_2 + 8 \vec{S}_1 \times \vec{v}_1 \cdot \vec{v}_2 \hat{n} \cdot \vec{v}_2 \vec{v}_1 \cdot \vec{v}_2 + \\
& 2 \hat{n} \times \vec{S}_1 \cdot \vec{v}_2 \vec{v}_1 \cdot \vec{v}_1 \vec{v}_1 \cdot \vec{v}_2 - 2 \hat{n} \times \vec{S}_1 \cdot \vec{v}_2 \vec{v}_1 \cdot \vec{v}_1 \vec{v}_2 \cdot \vec{v}_2 - \hat{n} \times \vec{S}_1 \cdot \vec{v}_1 \vec{v}_1 \cdot \vec{v}_2 \vec{v}_2 \cdot \vec{v}_2 \Big) m_1 m_2 G^2 + \\
& r m_1 m_2 \left( 2 \log \left( \frac{r}{R_\theta} \right) \hat{n} \times \vec{S}_1 \cdot \vec{a}_2 - \frac{\hat{n} \times \vec{S}_1 \cdot \vec{a}_2}{\epsilon_d} - \hat{n} \times \vec{S}_1 \cdot \vec{a}_2 \right) G^2 + \\
& m_1 m_2 \left( -\frac{2}{3} \log \left( \frac{r}{R_\theta} \right) \vec{S}_1 \times \vec{a}_1 \cdot \vec{a}_2 + \frac{5}{18} \vec{S}_1 \times \vec{a}_1 \cdot \vec{a}_2 + \frac{31}{18} \vec{S}_1 \times \vec{v}_1 \cdot \vec{a}_2 + \frac{5}{18} \vec{S}_1 \times \vec{v}_1 \cdot \vec{a}_2 - \vec{S}_1 \times \vec{v}_2 \cdot \vec{a}_2 + \right. \\
& \frac{13}{18} \vec{S}_1 \times \vec{a}_1 \cdot \vec{a}_2 + \frac{1}{6} \hat{n} \times \vec{S}_1 \cdot \vec{v}_1 \hat{n} \cdot \vec{a}_2 + \frac{1}{6} \hat{n} \times \vec{S}_1 \cdot \vec{a}_1 \hat{n} \cdot \vec{a}_2 + \hat{n} \times \vec{S}_1 \cdot \vec{a}_2 \hat{n} \cdot \vec{a}_1 + \hat{n} \times \vec{S}_1 \cdot \vec{a}_2 \hat{n} \cdot \vec{a}_1 - \\
& \frac{1}{6} \hat{n} \times \vec{S}_1 \cdot \vec{a}_1 \hat{n} \cdot \vec{a}_2 - \frac{1}{6} \hat{n} \times \vec{S}_1 \cdot \vec{v}_1 \hat{n} \cdot \vec{a}_2 - 2 \hat{n} \times \vec{S}_1 \cdot \vec{v}_2 \hat{n} \cdot \vec{a}_2 + 3 \hat{n} \times \vec{S}_1 \cdot \vec{a}_2 \hat{n} \cdot \vec{v}_1 + \hat{n} \times \vec{S}_1 \cdot \vec{a}_2 \hat{n} \cdot \vec{v}_1 - \\
& 4 \hat{n} \times \vec{S}_1 \cdot \vec{a}_2 \hat{n} \cdot \vec{v}_2 - \frac{10}{3} \vec{S}_1 \times \vec{v}_1 \cdot \vec{a}_2 \log \left( \frac{r}{R_\theta} \right) - \frac{2}{3} \vec{S}_1 \times \vec{v}_1 \cdot \vec{a}_2 \log \left( \frac{r}{R_\theta} \right) + 2 \vec{S}_1 \times \vec{v}_2 \cdot \vec{a}_2 \log \left( \frac{r}{R_\theta} \right) - \\
& \left. \frac{4}{3} \vec{S}_1 \times \vec{a}_1 \cdot \vec{a}_2 \log \left( \frac{r}{R_\theta} \right) + \frac{\frac{1}{3} \vec{S}_1 \times \vec{a}_1 \cdot \vec{a}_2 + \frac{5}{3} \vec{S}_1 \times \vec{v}_1 \cdot \vec{a}_2 + \frac{1}{3} \vec{S}_1 \times \vec{v}_1 \cdot \vec{a}_2 - \vec{S}_1 \times \vec{v}_2 \cdot \vec{a}_2 + \frac{2}{3} \vec{S}_1 \times \vec{a}_1 \cdot \vec{a}_2}{\epsilon_d} \right) G^2 \Big\}
\end{aligned}$$

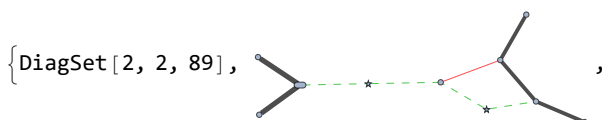

$$\begin{aligned}
& \frac{1}{r} G^2 \left( \frac{8}{3} \hat{n} \times \vec{a}_2 \cdot \vec{S}_1 (\hat{n} \cdot \vec{v}_1)^2 - \frac{8}{3} \vec{a}_2 \times \vec{S}_1 \cdot \vec{v}_1 \hat{n} \cdot \vec{v}_1 - \frac{2}{3} \vec{a}_2 \times \vec{S}_1 \cdot \vec{v}_2 \hat{n} \cdot \vec{v}_1 + \frac{8}{3} \vec{a}_2 \times \vec{S}_1 \cdot \vec{v}_2 \hat{n} \cdot \vec{v}_1 + \right. \\
& \quad \frac{4}{3} \hat{n} \times \vec{S}_1 \cdot \vec{v}_2 \hat{n} \cdot \vec{a}_2 \hat{n} \cdot \vec{v}_1 + \frac{8}{3} \hat{n} \times \vec{S}_1 \cdot \vec{v}_2 \hat{n} \cdot \vec{a}_2 \hat{n} \cdot \vec{v}_1 - \frac{4}{3} \hat{n} \times \vec{a}_2 \cdot \vec{S}_1 \hat{n} \cdot \vec{a}_2 \hat{n} \cdot \vec{v}_1 - 8 \hat{n} \times \vec{a}_2 \cdot \vec{S}_1 \hat{n} \cdot \vec{v}_2 \hat{n} \cdot \vec{v}_1 - \\
& \quad \frac{4}{3} \hat{n} \times \vec{S}_1 \cdot \vec{v}_2 (\hat{n} \cdot \vec{v}_2)^2 + \frac{1}{3} \hat{n} \times \vec{a}_2 \cdot \vec{S}_1 (\hat{n} \cdot \vec{v}_2)^2 + \frac{2}{3} \vec{S}_1 \times \vec{v}_1 \cdot \vec{v}_2 \hat{n} \cdot \vec{a}_2 + \frac{4}{3} \vec{a}_2 \times \vec{S}_1 \cdot \vec{v}_2 \hat{n} \cdot \vec{a}_1 + \\
& \quad \frac{4}{3} \vec{S}_1 \times \vec{v}_1 \cdot \vec{v}_2 \hat{n} \cdot \vec{a}_2 - \frac{2}{3} \vec{a}_1 \times \vec{S}_1 \cdot \vec{v}_2 \hat{n} \cdot \vec{a}_2 + \frac{2}{3} \vec{a}_2 \times \vec{S}_1 \cdot \vec{v}_1 \hat{n} \cdot \vec{a}_2 + \frac{4}{3} \hat{n} \times \vec{S}_1 \cdot \vec{v}_2 \hat{n} \cdot \vec{a}_1 \hat{n} \cdot \vec{a}_2 + 2 \vec{a}_1 \times \vec{a}_2 \cdot \vec{S}_1 \hat{n} \cdot \vec{v}_2 + \\
& \quad 4 \vec{a}_2 \times \vec{S}_1 \cdot \vec{v}_1 \hat{n} \cdot \vec{v}_2 + \frac{2}{3} \vec{a}_2 \times \vec{S}_1 \cdot \vec{v}_2 \hat{n} \cdot \vec{v}_2 - 4 \hat{n} \times \vec{a}_2 \cdot \vec{S}_1 \hat{n} \cdot \vec{a}_1 \hat{n} \cdot \vec{v}_2 - 2 \hat{n} \times \vec{S}_1 \cdot \vec{v}_2 \hat{n} \cdot \vec{a}_2 \hat{n} \cdot \vec{v}_2 - \\
& \quad \frac{2}{3} \hat{n} \times \vec{S}_1 \cdot \vec{v}_2 \vec{a}_2 \cdot \vec{v}_1 - \frac{2}{3} \hat{n} \times \vec{S}_1 \cdot \vec{v}_2 \vec{a}_1 \cdot \vec{a}_2 + 2 \hat{n} \times \vec{a}_2 \cdot \vec{S}_1 \vec{a}_1 \cdot \vec{v}_2 - \frac{4}{3} \hat{n} \times \vec{S}_1 \cdot \vec{v}_2 \vec{a}_2 \cdot \vec{v}_1 + \frac{2}{3} \hat{n} \times \vec{a}_2 \cdot \vec{S}_1 \vec{a}_2 \cdot \vec{v}_1 - \\
& \quad \left. \frac{4}{3} \hat{n} \times \vec{a}_2 \cdot \vec{S}_1 \vec{v}_1 \cdot \vec{v}_1 + 4 \hat{n} \times \vec{a}_2 \cdot \vec{S}_1 \vec{v}_1 \cdot \vec{v}_2 + \frac{2}{3} \hat{n} \times \vec{S}_1 \cdot \vec{v}_2 \vec{v}_2 \cdot \vec{v}_2 + \frac{1}{3} \hat{n} \times \vec{a}_2 \cdot \vec{S}_1 \vec{v}_2 \cdot \vec{v}_2 \right) m_2^2 + \frac{1}{r^2} \\
& G^2 \left( -\frac{4}{3} \hat{n} \times \vec{S}_1 \cdot \vec{v}_2 (\hat{n} \cdot \vec{v}_2)^3 + \frac{8}{3} \vec{S}_1 \times \vec{v}_1 \cdot \vec{v}_2 (\hat{n} \cdot \vec{v}_2)^2 - \frac{4}{3} \vec{a}_1 \times \vec{S}_1 \cdot \vec{v}_2 (\hat{n} \cdot \vec{v}_2)^2 + \frac{1}{3} \vec{a}_2 \times \vec{S}_1 \cdot \vec{v}_1 (\hat{n} \cdot \vec{v}_2)^2 + \right. \\
& \quad \frac{16}{3} \hat{n} \times \vec{S}_1 \cdot \vec{v}_2 \hat{n} \cdot \vec{a}_1 (\hat{n} \cdot \vec{v}_2)^2 + \frac{32}{3} \hat{n} \times \vec{S}_1 \cdot \vec{v}_2 \hat{n} \cdot \vec{v}_1 (\hat{n} \cdot \vec{v}_2)^2 - \frac{4}{3} \hat{n} \times \vec{a}_2 \cdot \vec{S}_1 \hat{n} \cdot \vec{v}_1 (\hat{n} \cdot \vec{v}_2)^2 + \\
& \quad 16 \hat{n} \times \vec{a}_2 \cdot \vec{S}_1 (\hat{n} \cdot \vec{v}_1)^2 \hat{n} \cdot \vec{v}_2 + 2 \vec{S}_1 \times \vec{v}_1 \cdot \vec{v}_2 \hat{n} \cdot \vec{a}_2 \hat{n} \cdot \vec{v}_2 - 8 \vec{a}_2 \times \vec{S}_1 \cdot \vec{v}_1 \hat{n} \cdot \vec{v}_1 \hat{n} \cdot \vec{v}_2 - \frac{4}{3} \vec{a}_2 \times \vec{S}_1 \cdot \vec{v}_2 \hat{n} \cdot \vec{v}_1 \hat{n} \cdot \vec{v}_2 + \\
& \quad 8 \hat{n} \times \vec{S}_1 \cdot \vec{v}_2 \hat{n} \cdot \vec{a}_2 \hat{n} \cdot \vec{v}_1 \hat{n} \cdot \vec{v}_2 - \frac{8}{3} \hat{n} \times \vec{S}_1 \cdot \vec{v}_2 \vec{a}_1 \cdot \vec{v}_2 \hat{n} \cdot \vec{v}_2 - 2 \hat{n} \times \vec{S}_1 \cdot \vec{v}_2 \vec{a}_2 \cdot \vec{v}_1 \hat{n} \cdot \vec{v}_2 - \\
& \quad 4 \hat{n} \times \vec{a}_2 \cdot \vec{S}_1 \vec{v}_1 \cdot \vec{v}_1 \hat{n} \cdot \vec{v}_2 - \frac{16}{3} \hat{n} \times \vec{S}_1 \cdot \vec{v}_2 \vec{v}_1 \cdot \vec{v}_2 \hat{n} \cdot \vec{v}_2 + \frac{2}{3} \hat{n} \times \vec{a}_2 \cdot \vec{S}_1 \vec{v}_1 \cdot \vec{v}_2 \hat{n} \cdot \vec{v}_2 - \frac{8}{3} \vec{a}_2 \times \vec{S}_1 \cdot \vec{v}_2 (\hat{n} \cdot \vec{v}_1)^2 - \\
& \quad \frac{16}{3} \hat{n} \times \vec{S}_1 \cdot \vec{v}_2 \hat{n} \cdot \vec{a}_2 (\hat{n} \cdot \vec{v}_1)^2 - \frac{8}{3} \vec{S}_1 \times \vec{v}_1 \cdot \vec{v}_2 \hat{n} \cdot \vec{a}_2 \hat{n} \cdot \vec{v}_1 + \frac{4}{3} \vec{S}_1 \times \vec{v}_1 \cdot \vec{v}_2 \vec{a}_2 \cdot \vec{v}_1 + \frac{8}{3} \hat{n} \times \vec{S}_1 \cdot \vec{v}_2 \hat{n} \cdot \vec{v}_1 \vec{a}_2 \cdot \vec{v}_1 + \\
& \quad \frac{4}{3} \vec{a}_2 \times \vec{S}_1 \cdot \vec{v}_2 \vec{v}_1 \cdot \vec{v}_1 + \frac{4}{3} \hat{n} \times \vec{S}_1 \cdot \vec{v}_2 \hat{n} \cdot \vec{a}_2 \vec{v}_1 \cdot \vec{v}_1 + 4 \vec{a}_2 \times \vec{S}_1 \cdot \vec{v}_1 \vec{v}_1 \cdot \vec{v}_2 + \frac{2}{3} \vec{a}_2 \times \vec{S}_1 \cdot \vec{v}_2 \vec{v}_1 \cdot \vec{v}_2 - \\
& \quad 2 \hat{n} \times \vec{S}_1 \cdot \vec{v}_2 \hat{n} \cdot \vec{a}_2 \vec{v}_1 \cdot \vec{v}_2 - 8 \hat{n} \times \vec{a}_2 \cdot \vec{S}_1 \hat{n} \cdot \vec{v}_1 \vec{v}_1 \cdot \vec{v}_2 - \frac{4}{3} \vec{S}_1 \times \vec{v}_1 \cdot \vec{v}_2 \vec{v}_2 \cdot \vec{v}_2 + \frac{2}{3} \vec{a}_1 \times \vec{S}_1 \cdot \vec{v}_2 \vec{v}_2 \cdot \vec{v}_2 + \\
& \quad \left. \frac{1}{3} \vec{a}_2 \times \vec{S}_1 \cdot \vec{v}_1 \vec{v}_2 \cdot \vec{v}_2 - \frac{4}{3} \hat{n} \times \vec{S}_1 \cdot \vec{v}_2 \hat{n} \cdot \vec{a}_1 \vec{v}_2 \cdot \vec{v}_2 - \frac{8}{3} \hat{n} \times \vec{S}_1 \cdot \vec{v}_2 \hat{n} \cdot \vec{v}_1 \vec{v}_2 \cdot \vec{v}_2 - \frac{2}{3} \hat{n} \times \vec{a}_2 \cdot \vec{S}_1 \hat{n} \cdot \vec{v}_1 \vec{v}_2 \cdot \vec{v}_2 \right) m_2^2 + \\
& \frac{1}{r^3} G^2 \left( \frac{4}{3} \vec{S}_1 \times \vec{v}_1 \cdot \vec{v}_2 (\hat{n} \cdot \vec{v}_2)^3 + 8 \hat{n} \times \vec{S}_1 \cdot \vec{v}_2 \hat{n} \cdot \vec{v}_1 (\hat{n} \cdot \vec{v}_2)^3 - 32 \hat{n} \times \vec{S}_1 \cdot \vec{v}_2 (\hat{n} \cdot \vec{v}_1)^2 (\hat{n} \cdot \vec{v}_2)^2 - \right. \\
& \quad \frac{32}{3} \vec{S}_1 \times \vec{v}_1 \cdot \vec{v}_2 \hat{n} \cdot \vec{v}_1 (\hat{n} \cdot \vec{v}_2)^2 + \frac{16}{3} \hat{n} \times \vec{S}_1 \cdot \vec{v}_2 \vec{v}_1 \cdot \vec{v}_1 (\hat{n} \cdot \vec{v}_2)^2 - 4 \hat{n} \times \vec{S}_1 \cdot \vec{v}_2 \vec{v}_1 \cdot \vec{v}_2 (\hat{n} \cdot \vec{v}_2)^2 + \\
& \quad \frac{16}{3} \vec{S}_1 \times \vec{v}_1 \cdot \vec{v}_2 \vec{v}_1 \cdot \vec{v}_2 \hat{n} \cdot \vec{v}_2 + \frac{64}{3} \hat{n} \times \vec{S}_1 \cdot \vec{v}_2 \hat{n} \cdot \vec{v}_1 \vec{v}_1 \cdot \vec{v}_2 \hat{n} \cdot \vec{v}_2 - \frac{8}{3} \hat{n} \times \vec{S}_1 \cdot \vec{v}_2 (\vec{v}_1 \cdot \vec{v}_2)^2 + \\
& \quad \left. \frac{16}{3} \hat{n} \times \vec{S}_1 \cdot \vec{v}_2 (\hat{n} \cdot \vec{v}_1)^2 \vec{v}_2 \cdot \vec{v}_2 + \frac{8}{3} \vec{S}_1 \times \vec{v}_1 \cdot \vec{v}_2 \hat{n} \cdot \vec{v}_1 \vec{v}_2 \cdot \vec{v}_2 - \frac{4}{3} \hat{n} \times \vec{S}_1 \cdot \vec{v}_2 \vec{v}_1 \cdot \vec{v}_1 \vec{v}_2 \cdot \vec{v}_2 \right) m_2^2 + \\
& G^2 r \left( -\frac{4}{3} \log \left( \frac{r}{R_\theta} \right) \hat{n} \times \vec{a}_2 \cdot \vec{S}_1 + \frac{2 \hat{n} \times \vec{a}_2 \cdot \vec{S}_1}{3 \epsilon_d} + \frac{2}{9} \hat{n} \times \vec{a}_2 \cdot \vec{S}_1 \right) m_2^2 + \\
& G^2 \left( -\frac{8}{3} \log \left( \frac{r}{R_\theta} \right) \frac{1}{\vec{a}_2 \times \vec{S}_1} \cdot \vec{v}_1 + \frac{4}{9} \frac{1}{\vec{a}_2 \times \vec{S}_1} \cdot \vec{v}_1 + \frac{7}{9} \frac{1}{\vec{a}_2 \times \vec{S}_1} \cdot \vec{v}_2 + \frac{2}{9} \frac{1}{\vec{a}_1 \times \vec{a}_2 \cdot \vec{S}_1} - \frac{2}{9} \frac{1}{\vec{a}_2 \times \vec{S}_1} \cdot \vec{v}_2 - \right. \\
& \quad \frac{2}{3} \hat{n} \times \vec{S}_1 \cdot \vec{v}_2 \hat{n} \cdot \vec{a}_2 - \frac{4}{3} \hat{n} \times \vec{a}_2 \cdot \vec{S}_1 \hat{n} \cdot \vec{a}_1 - \frac{2}{3} \hat{n} \times \vec{S}_1 \cdot \vec{v}_2 \hat{n} \cdot \vec{a}_2 + \frac{2}{3} \hat{n} \times \vec{a}_2 \cdot \vec{S}_1 \hat{n} \cdot \vec{a}_2 - \\
& \quad \left. \frac{8}{3} \hat{n} \times \vec{a}_2 \cdot \vec{S}_1 \hat{n} \cdot \vec{v}_1 + 2 \hat{n} \times \vec{a}_2 \cdot \vec{S}_1 \hat{n} \cdot \vec{v}_2 - \frac{2}{3} \frac{1}{\vec{a}_2 \times \vec{S}_1} \cdot \vec{v}_2 \log \left( \frac{r}{R_\theta} \right) - \frac{4}{3} \frac{1}{\vec{a}_1 \times \vec{a}_2 \cdot \vec{S}_1} \log \left( \frac{r}{R_\theta} \right) + \right.
\end{aligned}$$



$$\frac{4}{3} \vec{a}_2 \times \vec{S}_1 \cdot \vec{v}_2 \log \left( \frac{r}{R_\theta} \right) + \frac{\frac{4}{3} \vec{a}_2 \times \vec{S}_1 \cdot \vec{v}_1 + \frac{1}{3} \vec{a}_2 \times \vec{S}_1 \cdot \vec{v}_2 + \frac{2}{3} \vec{a}_1 \times \vec{a}_2 \cdot \vec{S}_1 - \frac{2}{3} \vec{a}_2 \times \vec{S}_1 \cdot \vec{v}_2}{\epsilon_d} m_2^2 \Bigg\}$$

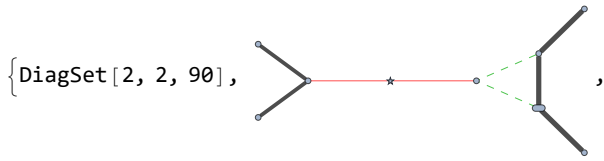

$$\begin{aligned} & \frac{1}{r^2} G^2 m_1 m_2 \left( -16 \hat{n} \cdot \vec{v}_1 \hat{n} \cdot \vec{v}_2 \vec{S}_1 \times \vec{v}_1 \cdot \vec{a}_1 + 16 \vec{v}_1 \cdot \vec{a}_1 \hat{n} \cdot \vec{v}_2 \hat{n} \times \vec{S}_1 \cdot \vec{v}_1 + 8 \vec{v}_1 \cdot \vec{v}_1 \hat{n} \cdot \vec{v}_2 \hat{n} \times \vec{S}_1 \cdot \vec{a}_1 + 3 \vec{v}_2 \cdot \vec{v}_2 \hat{n} \cdot \vec{v}_2 \hat{n} \times \vec{S}_1 \cdot \vec{a}_1 - \right. \\ & 6 \vec{v}_2 \cdot \vec{a}_2 \hat{n} \cdot \vec{v}_1 \hat{n} \times \vec{S}_1 \cdot \vec{v}_1 - 8 \vec{v}_1 \cdot \vec{a}_1 \vec{S}_1 \times \vec{v}_1 \cdot \vec{v}_2 - 4 \vec{v}_1 \cdot \vec{v}_1 \vec{S}_1 \times \vec{a}_1 \cdot \vec{v}_2 + 8 \vec{v}_1 \cdot \vec{v}_2 \vec{S}_1 \times \vec{v}_1 \cdot \vec{a}_1 - \frac{3}{2} \vec{v}_2 \cdot \vec{v}_2 \vec{S}_1 \times \vec{a}_1 \cdot \vec{v}_2 + \\ & \left. 8 \vec{v}_1 \cdot \vec{v}_1 \hat{n} \cdot \vec{v}_2 \hat{n} \times \vec{S}_1 \cdot \vec{v}_1 + 3 \vec{v}_2 \cdot \vec{v}_2 \hat{n} \cdot \vec{v}_2 \hat{n} \times \vec{S}_1 \cdot \vec{v}_1 - 4 \vec{v}_1 \cdot \vec{v}_1 \vec{S}_1 \times \vec{v}_1 \cdot \vec{v}_2 - \frac{3}{2} \vec{v}_2 \cdot \vec{v}_2 \vec{S}_1 \times \vec{v}_1 \cdot \vec{v}_2 \right) + \\ & \frac{1}{r} G^2 m_1 m_2 \left( 8 \hat{n} \cdot \vec{v}_2 \vec{S}_1 \times \vec{v}_1 \cdot \vec{a}_1 + 8 \hat{n} \cdot \vec{v}_2 \vec{S}_1 \times \vec{v}_1 \cdot \vec{a}_1 + 3 \vec{v}_2 \cdot \vec{a}_2 \hat{n} \times \vec{S}_1 \cdot \vec{v}_1 + 3 \vec{v}_2 \cdot \vec{a}_2 \hat{n} \times \vec{S}_1 \cdot \vec{a}_1 \right) + \frac{1}{r^3} \\ & G^2 m_1 m_2 \left( 8 \vec{v}_1 \cdot \vec{v}_1 \hat{n} \cdot \vec{v}_1 \vec{S}_1 \times \vec{v}_1 \cdot \vec{v}_2 - 32 \vec{v}_1 \cdot \vec{v}_1 \hat{n} \cdot \vec{v}_1 \hat{n} \cdot \vec{v}_2 \hat{n} \times \vec{S}_1 \cdot \vec{v}_1 + 8 \vec{v}_1 \cdot \vec{v}_2 \vec{v}_1 \cdot \vec{v}_1 \hat{n} \times \vec{S}_1 \cdot \vec{v}_1 + \right. \\ & \left. 3 \vec{v}_2 \cdot \vec{v}_2 \hat{n} \cdot \vec{v}_1 \vec{S}_1 \times \vec{v}_1 \cdot \vec{v}_2 - 12 \vec{v}_2 \cdot \vec{v}_2 \hat{n} \cdot \vec{v}_1 \hat{n} \cdot \vec{v}_2 \hat{n} \times \vec{S}_1 \cdot \vec{v}_1 + 3 \vec{v}_1 \cdot \vec{v}_2 \vec{v}_2 \cdot \vec{v}_2 \hat{n} \times \vec{S}_1 \cdot \vec{v}_1 \right) \Bigg\} \end{aligned}$$

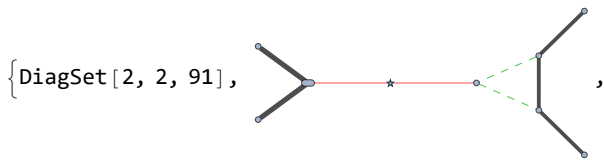

$$\begin{aligned} & \frac{1}{r^2} G^2 m_2^2 \left( -32 \vec{a}_2 \cdot \vec{v}_2 \hat{n} \cdot \vec{v}_1 \hat{n} \times \vec{S}_1 \cdot \vec{v}_1 - 16 \vec{v}_2 \cdot \vec{v}_2 \hat{n} \cdot \vec{v}_2 \hat{n} \times \vec{a}_1 \cdot \vec{S}_1 + 8 \vec{v}_2 \cdot \vec{v}_2 \vec{a}_1 \times \vec{S}_1 \cdot \vec{v}_2 + \right. \\ & \left. 16 \vec{v}_2 \cdot \vec{v}_2 \hat{n} \cdot \vec{v}_2 \hat{n} \times \vec{S}_1 \cdot \vec{v}_1 - 8 \vec{v}_2 \cdot \vec{v}_2 \vec{S}_1 \times \vec{v}_1 \cdot \vec{v}_2 \right) + \frac{G^2 m_2^2 \left( 16 \vec{a}_2 \cdot \vec{v}_2 \hat{n} \times \vec{S}_1 \cdot \vec{v}_1 - 16 \vec{a}_2 \cdot \vec{v}_2 \hat{n} \times \vec{a}_1 \cdot \vec{S}_1 \right)}{r} + \\ & \frac{1}{r^3} G^2 m_2^2 \left( 16 \vec{v}_2 \cdot \vec{v}_2 \hat{n} \cdot \vec{v}_1 \vec{S}_1 \times \vec{v}_1 \cdot \vec{v}_2 - 64 \vec{v}_2 \cdot \vec{v}_2 \hat{n} \cdot \vec{v}_1 \hat{n} \cdot \vec{v}_2 \hat{n} \times \vec{S}_1 \cdot \vec{v}_1 + 16 \vec{v}_1 \cdot \vec{v}_2 \vec{v}_2 \cdot \vec{v}_2 \hat{n} \times \vec{S}_1 \cdot \vec{v}_1 \right) \Bigg\} \end{aligned}$$

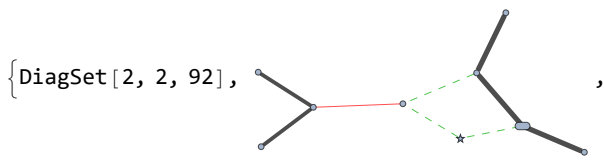

$$\begin{aligned} & \frac{1}{r} \left( -7 \vec{S}_1 \times \vec{v}_1 \cdot \vec{a}_1 \hat{n} \cdot \vec{a}_1 + 21 \vec{S}_1 \times \vec{v}_1 \cdot \vec{a}_1 \hat{n} \cdot \vec{v}_1 + 12 \vec{S}_1 \times \vec{v}_1 \cdot \vec{a}_1 \hat{n} \cdot \vec{v}_1 - 16 \vec{S}_1 \times \vec{v}_1 \cdot \vec{a}_1 \hat{n} \cdot \vec{v}_2 - \right. \\ & 8 \vec{S}_1 \times \vec{v}_1 \cdot \vec{a}_1 \hat{n} \cdot \vec{v}_2 - \hat{n} \times \vec{S}_1 \cdot \vec{v}_1 \vec{a}_1 \cdot \vec{a}_1 - 3 \hat{n} \times \vec{S}_1 \cdot \vec{v}_1 \vec{v}_1 \cdot \vec{a}_1 - 5 \hat{n} \times \vec{S}_1 \cdot \vec{a}_1 \vec{v}_1 \cdot \vec{a}_1 + 9 \hat{n} \times \vec{S}_1 \cdot \vec{a}_1 \vec{v}_1 \cdot \vec{v}_1 + \\ & \left. 4 \hat{n} \times \vec{S}_1 \cdot \vec{v}_1 \vec{v}_1 \cdot \vec{v}_1 + 4 \hat{n} \times \vec{S}_1 \cdot \vec{a}_1 \vec{v}_1 \cdot \vec{v}_1 + 6 \hat{n} \times \vec{S}_1 \cdot \vec{v}_1 \vec{v}_2 \cdot \vec{a}_2 + 3 \hat{n} \times \vec{S}_1 \cdot \vec{a}_1 \vec{v}_2 \cdot \vec{v}_2 \right) m_1 m_2 G^2 + \frac{1}{r^2} \\ & \left( \frac{7}{2} \vec{S}_1 \times \vec{v}_1 \cdot \vec{a}_1 (\hat{n} \cdot \vec{v}_1)^2 - 2 \vec{S}_1 \times \vec{v}_1 \cdot \vec{a}_1 \hat{n} \cdot \vec{v}_2 \hat{n} \cdot \vec{v}_1 + \frac{9}{2} \hat{n} \times \vec{S}_1 \cdot \vec{v}_1 \vec{v}_1 \cdot \vec{a}_1 \hat{n} \cdot \vec{v}_1 + 2 \hat{n} \times \vec{S}_1 \cdot \vec{v}_1 \vec{v}_1 \cdot \vec{v}_1 \hat{n} \cdot \vec{v}_1 + \right. \\ & \frac{7}{2} \hat{n} \times \vec{S}_1 \cdot \vec{a}_1 \vec{v}_1 \cdot \vec{v}_1 \hat{n} \cdot \vec{v}_1 - 3 \hat{n} \times \vec{S}_1 \cdot \vec{v}_1 \vec{v}_2 \cdot \vec{a}_2 \hat{n} \cdot \vec{v}_1 - \frac{9}{2} \hat{n} \times \vec{S}_1 \cdot \vec{v}_1 \vec{v}_2 \cdot \vec{v}_2 \hat{n} \cdot \vec{v}_1 + \vec{S}_1 \times \vec{v}_1 \cdot \vec{v}_2 \vec{v}_1 \cdot \vec{a}_1 - \\ & 2 \hat{n} \times \vec{S}_1 \cdot \vec{v}_1 \hat{n} \cdot \vec{v}_2 \vec{v}_1 \cdot \vec{a}_1 + 4 \vec{S}_1 \times \vec{v}_1 \cdot \vec{v}_2 \vec{v}_1 \cdot \vec{v}_1 + 5 \vec{S}_1 \times \vec{a}_1 \cdot \vec{v}_2 \vec{v}_1 \cdot \vec{v}_1 + 8 \vec{S}_1 \times \vec{v}_1 \cdot \vec{a}_1 \vec{v}_1 \cdot \vec{v}_1 - \\ & \left. 4 \hat{n} \times \vec{S}_1 \cdot \vec{v}_1 \hat{n} \cdot \vec{a}_1 \vec{v}_1 \cdot \vec{v}_1 - 8 \hat{n} \times \vec{S}_1 \cdot \vec{v}_1 \hat{n} \cdot \vec{v}_2 \vec{v}_1 \cdot \vec{v}_1 - 10 \hat{n} \times \vec{S}_1 \cdot \vec{a}_1 \hat{n} \cdot \vec{v}_2 \vec{v}_1 \cdot \vec{v}_1 + \vec{S}_1 \times \vec{v}_1 \cdot \vec{a}_1 \vec{v}_1 \cdot \vec{v}_2 - \right. \end{aligned}$$

$$\begin{aligned}
& 3 \frac{1}{S_1} \times \vec{v}_1 \cdot \vec{v}_2 \vec{v}_2 \cdot \vec{v}_2 - \frac{3}{2} \vec{S}_1 \times \vec{v}_1 \cdot \vec{a}_1 \vec{v}_2 \cdot \vec{v}_2 - \frac{3}{2} \hat{n} \times \vec{S}_1 \cdot \vec{v}_1 \hat{n} \cdot \vec{a}_1 \vec{v}_2 \cdot \vec{v}_2 + 6 \hat{n} \times \vec{S}_1 \cdot \vec{v}_1 \hat{n} \cdot \vec{v}_2 \vec{v}_2 \cdot \vec{v}_2 \Big) m_1 m_2 G^2 + \\
& \frac{1}{r^3} \left( 3 \hat{n} \times \vec{S}_1 \cdot \vec{v}_1 \vec{v}_2 \cdot \vec{v}_2 (\hat{n} \cdot \vec{v}_1)^2 - 2 \vec{S}_1 \times \vec{v}_1 \cdot \vec{v}_2 \vec{v}_1 \cdot \vec{v}_1 \hat{n} \cdot \vec{v}_1 + 8 \hat{n} \times \vec{S}_1 \cdot \vec{v}_1 \hat{n} \cdot \vec{v}_2 \vec{v}_1 \cdot \vec{v}_1 \hat{n} \cdot \vec{v}_1 + \right. \\
& \quad \frac{3}{2} \vec{S}_1 \times \vec{v}_1 \cdot \vec{v}_2 \vec{v}_2 \cdot \vec{v}_2 \hat{n} \cdot \vec{v}_1 - 6 \hat{n} \times \vec{S}_1 \cdot \vec{v}_1 \hat{n} \cdot \vec{v}_2 \vec{v}_2 \cdot \vec{v}_2 \hat{n} \cdot \vec{v}_1 + 2 \hat{n} \times \vec{S}_1 \cdot \vec{v}_1 (\vec{v}_1 \cdot \vec{v}_1)^2 - \\
& \quad \left. 2 \hat{n} \times \vec{S}_1 \cdot \vec{v}_1 \vec{v}_1 \cdot \vec{v}_1 \vec{v}_1 \cdot \vec{v}_2 - \frac{3}{2} \hat{n} \times \vec{S}_1 \cdot \vec{v}_1 \vec{v}_1 \cdot \vec{v}_1 \vec{v}_2 \cdot \vec{v}_2 + \frac{3}{2} \hat{n} \times \vec{S}_1 \cdot \vec{v}_1 \vec{v}_1 \cdot \vec{v}_2 \vec{v}_2 \cdot \vec{v}_2 \right) m_1 m_2 G^2 + \\
& m_1 m_2 \left( -8 \log \left( \frac{r}{R_\theta} \right) \frac{2}{S_1} \times \vec{v}_1 \cdot \vec{a}_1 + 8 \frac{2}{S_1} \times \vec{v}_1 \cdot \vec{a}_1 - 8 \vec{S}_1 \times \vec{a}_1 \cdot \frac{1}{a_1} + 8 \vec{S}_1 \times \vec{a}_1 \cdot \frac{1}{a_1} \log \left( \frac{r}{R_\theta} \right) + \frac{4 \frac{2}{S_1} \times \vec{v}_1 \cdot \vec{a}_1 - 4 \vec{S}_1 \times \vec{a}_1 \cdot \frac{1}{a_1}}{\epsilon_d} \right) G^2 \Big\}
\end{aligned}$$

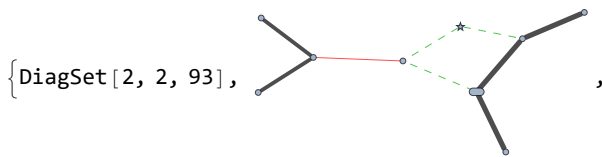

$$\begin{aligned}
& \frac{1}{r} \left( -9 \vec{S}_1 \times \vec{v}_1 \cdot \vec{a}_1 \hat{n} \cdot \vec{a}_1 - 5 \vec{S}_1 \times \vec{v}_1 \cdot \vec{a}_1 \hat{n} \cdot \vec{v}_1 + 4 \vec{S}_1 \times \vec{v}_1 \cdot \frac{1}{a_1} \hat{n} \cdot \vec{v}_1 + 8 \vec{S}_1 \times \vec{v}_1 \cdot \vec{a}_1 \hat{n} \cdot \vec{v}_2 - \right. \\
& \quad 7 \hat{n} \times \vec{S}_1 \cdot \vec{v}_1 \vec{a}_1 \cdot \vec{a}_1 - 13 \hat{n} \times \vec{S}_1 \cdot \vec{v}_1 \vec{v}_1 \cdot \vec{a}_1 - 11 \hat{n} \times \vec{S}_1 \cdot \vec{a}_1 \vec{v}_1 \cdot \vec{a}_1 + 7 \hat{n} \times \vec{S}_1 \cdot \vec{a}_1 \vec{v}_1 \cdot \vec{v}_1 + \\
& \quad \left. 4 \hat{n} \times \vec{S}_1 \cdot \vec{v}_1 \vec{v}_1 \cdot \vec{v}_1 + 4 \hat{n} \times \vec{S}_1 \cdot \frac{1}{a_1} \vec{v}_1 \cdot \vec{v}_1 - 6 \hat{n} \times \vec{S}_1 \cdot \vec{a}_1 \vec{v}_2 \cdot \vec{a}_2 - 3 \hat{n} \times \vec{S}_1 \cdot \vec{a}_1 \vec{v}_2 \cdot \vec{v}_2 \right) m_1 m_2 G^2 + \frac{1}{r^2} \\
& \left( \frac{9}{2} \vec{S}_1 \times \vec{v}_1 \cdot \vec{a}_1 (\hat{n} \cdot \vec{v}_1)^2 - 2 \vec{S}_1 \times \vec{v}_1 \cdot \vec{a}_1 \hat{n} \cdot \vec{v}_2 \hat{n} \cdot \vec{v}_1 + \frac{55}{2} \hat{n} \times \vec{S}_1 \cdot \vec{v}_1 \vec{v}_1 \cdot \vec{a}_1 \hat{n} \cdot \vec{v}_1 - 6 \hat{n} \times \vec{S}_1 \cdot \vec{v}_1 \vec{v}_1 \cdot \vec{v}_1 \hat{n} \cdot \vec{v}_1 - \right. \\
& \quad \frac{7}{2} \hat{n} \times \vec{S}_1 \cdot \vec{a}_1 \vec{v}_1 \cdot \vec{v}_1 \hat{n} \cdot \vec{v}_1 + 3 \hat{n} \times \vec{S}_1 \cdot \vec{v}_1 \vec{v}_2 \cdot \vec{a}_2 \hat{n} \cdot \vec{v}_1 + \frac{3}{2} \hat{n} \times \vec{S}_1 \cdot \vec{v}_1 \vec{v}_2 \cdot \vec{v}_2 \hat{n} \cdot \vec{v}_1 + 9 \hat{n} \times \vec{S}_1 \cdot \vec{a}_1 \vec{v}_2 \cdot \vec{v}_2 \hat{n} \cdot \vec{v}_1 + \\
& \quad 9 \vec{S}_1 \times \vec{v}_1 \cdot \vec{v}_2 \vec{v}_1 \cdot \vec{a}_1 - 18 \hat{n} \times \vec{S}_1 \cdot \vec{v}_1 \hat{n} \cdot \vec{v}_2 \vec{v}_1 \cdot \vec{a}_1 - 4 \frac{1}{S_1} \times \vec{v}_1 \cdot \vec{v}_2 \vec{v}_1 \cdot \vec{v}_1 - 3 \vec{S}_1 \times \vec{a}_1 \cdot \vec{v}_2 \vec{v}_1 \cdot \vec{v}_1 + 8 \vec{S}_1 \times \vec{v}_1 \cdot \vec{a}_1 \vec{v}_1 \cdot \vec{v}_1 - \\
& \quad 12 \hat{n} \times \vec{S}_1 \cdot \vec{v}_1 \hat{n} \cdot \vec{a}_1 \vec{v}_1 \cdot \vec{v}_1 + 8 \hat{n} \times \vec{S}_1 \cdot \vec{v}_1 \hat{n} \cdot \vec{v}_2 \vec{v}_1 \cdot \vec{v}_1 + 6 \hat{n} \times \vec{S}_1 \cdot \vec{a}_1 \hat{n} \cdot \vec{v}_2 \vec{v}_1 \cdot \vec{v}_1 + \vec{S}_1 \times \vec{v}_1 \cdot \vec{a}_1 \vec{v}_1 \cdot \vec{v}_2 + \\
& \quad \left. 3 \vec{S}_1 \times \vec{a}_1 \cdot \vec{v}_2 \vec{v}_2 \cdot \vec{v}_2 + \frac{9}{2} \vec{S}_1 \times \vec{v}_1 \cdot \vec{a}_1 \vec{v}_2 \cdot \vec{v}_2 - \frac{9}{2} \hat{n} \times \vec{S}_1 \cdot \vec{v}_1 \hat{n} \cdot \vec{a}_1 \vec{v}_2 \cdot \vec{v}_2 - 6 \hat{n} \times \vec{S}_1 \cdot \vec{a}_1 \hat{n} \cdot \vec{v}_2 \vec{v}_2 \cdot \vec{v}_2 \right) m_1 m_2 G^2 + \\
& \frac{1}{r^3} \left( 8 \hat{n} \times \vec{S}_1 \cdot \vec{v}_1 \vec{v}_1 \cdot \vec{v}_1 (\hat{n} \cdot \vec{v}_1)^2 - 3 \hat{n} \times \vec{S}_1 \cdot \vec{v}_1 \vec{v}_2 \cdot \vec{v}_2 (\hat{n} \cdot \vec{v}_1)^2 + 2 \vec{S}_1 \times \vec{v}_1 \cdot \vec{v}_2 \vec{v}_1 \cdot \vec{v}_1 \hat{n} \cdot \vec{v}_1 - \right. \\
& \quad 8 \hat{n} \times \vec{S}_1 \cdot \vec{v}_1 \hat{n} \cdot \vec{v}_2 \vec{v}_1 \cdot \vec{v}_1 \hat{n} \cdot \vec{v}_1 - \frac{3}{2} \vec{S}_1 \times \vec{v}_1 \cdot \vec{v}_2 \vec{v}_2 \cdot \vec{v}_2 \hat{n} \cdot \vec{v}_1 + 6 \hat{n} \times \vec{S}_1 \cdot \vec{v}_1 \hat{n} \cdot \vec{v}_2 \vec{v}_2 \cdot \vec{v}_2 \hat{n} \cdot \vec{v}_1 + 2 \hat{n} \times \vec{S}_1 \cdot \vec{v}_1 (\vec{v}_1 \cdot \vec{v}_1)^2 + \\
& \quad \left. 2 \hat{n} \times \vec{S}_1 \cdot \vec{v}_1 \vec{v}_1 \cdot \vec{v}_1 \vec{v}_1 \cdot \vec{v}_2 + \frac{3}{2} \hat{n} \times \vec{S}_1 \cdot \vec{v}_1 \vec{v}_1 \cdot \vec{v}_1 \vec{v}_2 \cdot \vec{v}_2 - \frac{3}{2} \hat{n} \times \vec{S}_1 \cdot \vec{v}_1 \vec{v}_1 \cdot \vec{v}_2 \vec{v}_2 \cdot \vec{v}_2 \right) m_1 m_2 G^2 + \\
& m_1 m_2 \left( -8 \log \left( \frac{r}{R_\theta} \right) \frac{2}{S_1} \times \vec{v}_1 \cdot \vec{a}_1 + 8 \frac{2}{S_1} \times \vec{v}_1 \cdot \vec{a}_1 - 8 \vec{S}_1 \times \vec{a}_1 \cdot \frac{1}{a_1} + 8 \vec{S}_1 \times \vec{a}_1 \cdot \frac{1}{a_1} \log \left( \frac{r}{R_\theta} \right) + \frac{4 \frac{2}{S_1} \times \vec{v}_1 \cdot \vec{a}_1 - 4 \vec{S}_1 \times \vec{a}_1 \cdot \frac{1}{a_1}}{\epsilon_d} \right) G^2 \Big\}
\end{aligned}$$

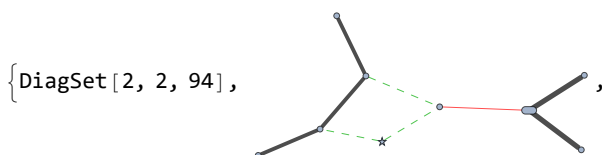

$$\begin{aligned}
& \frac{1}{r^2} G^2 m_2^2 \left( 32 \vec{a}_2 \cdot \vec{v}_2 \hat{n} \cdot \vec{v}_1 \hat{n} \times \vec{S}_1 \cdot \vec{v}_1 - 64 \vec{a}_2 \cdot \vec{v}_2 \hat{n} \cdot \vec{v}_2 \hat{n} \times \vec{S}_1 \cdot \vec{v}_1 + 32 \vec{v}_2 \cdot \vec{v}_2 \hat{n} \cdot \vec{a}_2 \hat{n} \times \vec{S}_1 \cdot \vec{v}_1 + 32 \vec{a}_2 \cdot \vec{v}_2 \vec{S}_1 \times \vec{v}_1 \cdot \vec{v}_2 - \right. \\
& \quad \left. 16 \vec{v}_2 \cdot \vec{v}_2 \vec{a}_2 \times \vec{S}_1 \cdot \vec{v}_1 \right) + \frac{G^2 m_2^2 \left( -16 \vec{a}_2 \cdot \vec{a}_2 \hat{n} \times \vec{S}_1 \cdot \vec{v}_1 - 16 \vec{a}_2 \cdot \vec{v}_2 \hat{n} \times \frac{1}{S_1} \cdot \vec{v}_1 + 16 \vec{a}_2 \cdot \vec{v}_2 \hat{n} \times \vec{a}_1 \cdot \vec{S}_1 \right)}{r} +
\end{aligned}$$

$$\frac{1}{r^3} G^2 m_2^2 \left( 16 \vec{v}_2 \cdot \vec{v}_2 (\hat{n} \cdot \vec{v}_2)^2 \hat{n} \times \vec{S}_1 \cdot \vec{v}_1 - 8 \vec{v}_2 \cdot \vec{v}_2 \hat{n} \cdot \vec{v}_2 \vec{S}_1 \times \vec{v}_1 \cdot \vec{v}_2 + 8 (\vec{v}_2 \cdot \vec{v}_2)^2 \hat{n} \times \vec{S}_1 \cdot \vec{v}_1 \right) \Big\}$$

$$\left\{ \text{DiagSet}[2, 2, 95], \right.$$
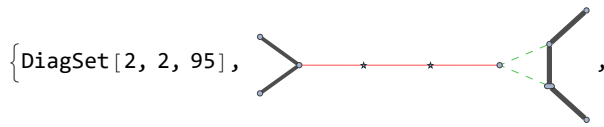

$$,$$

$$\begin{aligned} & \frac{1}{r} \left( \frac{4}{3} \hat{n} \times \vec{S}_1 \cdot \vec{a}_1 (\hat{n} \cdot \vec{v}_2)^2 + \frac{2}{3} \hat{n} \times \vec{S}_1 \cdot \vec{v}_1 (\hat{n} \cdot \vec{v}_2)^2 + \frac{2}{3} \hat{n} \times \vec{S}_1 \cdot \vec{a}_1 (\hat{n} \cdot \vec{v}_2)^2 - \frac{4}{3} \vec{S}_1 \times \vec{a}_1 \cdot \vec{v}_2 \hat{n} \cdot \vec{v}_2 - \frac{2}{3} \vec{S}_1 \times \vec{v}_1 \cdot \vec{v}_2 \hat{n} \cdot \vec{v}_2 - \right. \\ & \quad \frac{2}{3} \vec{S}_1 \times \vec{a}_1 \cdot \vec{v}_2 \hat{n} \cdot \vec{v}_2 + \frac{1}{3} \vec{S}_1 \times \vec{v}_1 \cdot \vec{a}_2 \hat{n} \cdot \vec{a}_1 - \frac{1}{3} \vec{S}_1 \times \vec{v}_1 \cdot \vec{a}_1 \hat{n} \cdot \vec{a}_2 - \frac{2}{3} \hat{n} \times \vec{S}_1 \cdot \vec{v}_1 \hat{n} \cdot \vec{a}_1 \hat{n} \cdot \vec{a}_2 + \frac{2}{3} \vec{S}_1 \times \vec{v}_1 \cdot \vec{a}_2 \hat{n} \cdot \vec{v}_1 + \\ & \quad \frac{2}{3} \vec{S}_1 \times \vec{a}_1 \cdot \vec{a}_2 \hat{n} \cdot \vec{v}_1 - \frac{4}{3} \hat{n} \times \vec{S}_1 \cdot \vec{v}_1 \hat{n} \cdot \vec{a}_2 \hat{n} \cdot \vec{v}_1 - \frac{4}{3} \hat{n} \times \vec{S}_1 \cdot \vec{a}_1 \hat{n} \cdot \vec{a}_2 \hat{n} \cdot \vec{v}_1 + \frac{1}{3} \hat{n} \times \vec{S}_1 \cdot \vec{v}_1 \vec{a}_1 \cdot \vec{a}_2 + \\ & \quad \left. \frac{2}{3} \hat{n} \times \vec{S}_1 \cdot \vec{v}_1 \vec{v}_1 \cdot \vec{a}_2 + \frac{2}{3} \hat{n} \times \vec{S}_1 \cdot \vec{a}_1 \vec{v}_1 \cdot \vec{a}_2 - \frac{2}{3} \hat{n} \times \vec{S}_1 \cdot \vec{a}_1 \vec{v}_2 \cdot \vec{v}_2 - \frac{1}{3} \hat{n} \times \vec{S}_1 \cdot \vec{v}_1 \vec{v}_2 \cdot \vec{v}_2 - \frac{1}{3} \hat{n} \times \vec{S}_1 \cdot \vec{a}_1 \vec{v}_2 \cdot \vec{v}_2 \right) m_1 m_2 G^2 + \\ & \frac{1}{r^2} \left( -\frac{2}{3} \vec{S}_1 \times \vec{v}_1 \cdot \vec{a}_2 (\hat{n} \cdot \vec{v}_1)^2 + \frac{8}{3} \hat{n} \times \vec{S}_1 \cdot \vec{v}_1 \hat{n} \cdot \vec{a}_2 (\hat{n} \cdot \vec{v}_1)^2 - \frac{16}{3} \hat{n} \times \vec{S}_1 \cdot \vec{v}_1 (\hat{n} \cdot \vec{v}_2)^2 \hat{n} \cdot \vec{v}_1 - \right. \\ & \quad \frac{16}{3} \hat{n} \times \vec{S}_1 \cdot \vec{a}_1 (\hat{n} \cdot \vec{v}_2)^2 \hat{n} \cdot \vec{v}_1 + \frac{8}{3} \vec{S}_1 \times \vec{v}_1 \cdot \vec{v}_2 \hat{n} \cdot \vec{v}_2 \hat{n} \cdot \vec{v}_1 + \frac{8}{3} \vec{S}_1 \times \vec{a}_1 \cdot \vec{v}_2 \hat{n} \cdot \vec{v}_2 \hat{n} \cdot \vec{v}_1 - \frac{4}{3} \hat{n} \times \vec{S}_1 \cdot \vec{v}_1 \vec{v}_1 \cdot \vec{a}_2 \hat{n} \cdot \vec{v}_1 + \\ & \quad \frac{4}{3} \hat{n} \times \vec{S}_1 \cdot \vec{v}_1 \vec{v}_2 \cdot \vec{v}_2 \hat{n} \cdot \vec{v}_1 + \frac{4}{3} \hat{n} \times \vec{S}_1 \cdot \vec{a}_1 \vec{v}_2 \cdot \vec{v}_2 \hat{n} \cdot \vec{v}_1 - \frac{2}{3} \vec{S}_1 \times \vec{v}_1 \cdot \vec{a}_1 (\hat{n} \cdot \vec{v}_2)^2 - \frac{8}{3} \hat{n} \times \vec{S}_1 \cdot \vec{v}_1 \hat{n} \cdot \vec{a}_1 (\hat{n} \cdot \vec{v}_2)^2 + \\ & \quad \frac{4}{3} \vec{S}_1 \times \vec{v}_1 \cdot \vec{v}_2 \hat{n} \cdot \vec{a}_1 \hat{n} \cdot \vec{v}_2 - \frac{2}{3} \vec{S}_1 \times \vec{v}_1 \cdot \vec{v}_2 \vec{a}_1 \cdot \vec{v}_2 + \frac{4}{3} \hat{n} \times \vec{S}_1 \cdot \vec{v}_1 \hat{n} \cdot \vec{v}_2 \vec{a}_1 \cdot \vec{v}_2 + \frac{1}{3} \vec{S}_1 \times \vec{v}_1 \cdot \vec{a}_2 \vec{v}_1 \cdot \vec{v}_1 - \\ & \quad \frac{2}{3} \hat{n} \times \vec{S}_1 \cdot \vec{v}_1 \hat{n} \cdot \vec{a}_2 \vec{v}_1 \cdot \vec{v}_1 - \frac{4}{3} \vec{S}_1 \times \vec{v}_1 \cdot \vec{v}_2 \vec{v}_1 \cdot \vec{v}_2 - \frac{4}{3} \vec{S}_1 \times \vec{a}_1 \cdot \vec{v}_2 \vec{v}_1 \cdot \vec{v}_2 + \frac{8}{3} \hat{n} \times \vec{S}_1 \cdot \vec{v}_1 \hat{n} \cdot \vec{v}_2 \vec{v}_1 \cdot \vec{v}_2 + \\ & \quad \left. \frac{8}{3} \hat{n} \times \vec{S}_1 \cdot \vec{a}_1 \hat{n} \cdot \vec{v}_2 \vec{v}_1 \cdot \vec{v}_2 + \frac{1}{3} \vec{S}_1 \times \vec{v}_1 \cdot \vec{a}_1 \vec{v}_2 \cdot \vec{v}_2 + \frac{2}{3} \hat{n} \times \vec{S}_1 \cdot \vec{v}_1 \hat{n} \cdot \vec{a}_1 \vec{v}_2 \cdot \vec{v}_2 \right) m_1 m_2 G^2 + \frac{1}{r^3} \\ & \left( 16 \hat{n} \times \vec{S}_1 \cdot \vec{v}_1 (\hat{n} \cdot \vec{v}_2)^2 (\hat{n} \cdot \vec{v}_1)^2 - \frac{16}{3} \vec{S}_1 \times \vec{v}_1 \cdot \vec{v}_2 \hat{n} \cdot \vec{v}_2 (\hat{n} \cdot \vec{v}_1)^2 - \frac{8}{3} \hat{n} \times \vec{S}_1 \cdot \vec{v}_1 \vec{v}_2 \cdot \vec{v}_2 (\hat{n} \cdot \vec{v}_1)^2 + \right. \\ & \quad \frac{8}{3} \vec{S}_1 \times \vec{v}_1 \cdot \vec{v}_2 \vec{v}_1 \cdot \vec{v}_2 \hat{n} \cdot \vec{v}_1 - \frac{32}{3} \hat{n} \times \vec{S}_1 \cdot \vec{v}_1 \hat{n} \cdot \vec{v}_2 \vec{v}_1 \cdot \vec{v}_2 \hat{n} \cdot \vec{v}_1 + \frac{4}{3} \hat{n} \times \vec{S}_1 \cdot \vec{v}_1 (\vec{v}_1 \cdot \vec{v}_2)^2 - \\ & \quad \left. \frac{8}{3} \hat{n} \times \vec{S}_1 \cdot \vec{v}_1 (\hat{n} \cdot \vec{v}_2)^2 \vec{v}_1 \cdot \vec{v}_1 + \frac{4}{3} \vec{S}_1 \times \vec{v}_1 \cdot \vec{v}_2 \hat{n} \cdot \vec{v}_2 \vec{v}_1 \cdot \vec{v}_1 + \frac{2}{3} \hat{n} \times \vec{S}_1 \cdot \vec{v}_1 \vec{v}_1 \cdot \vec{v}_1 \vec{v}_2 \cdot \vec{v}_2 \right) m_1 m_2 G^2 + \\ & m_1 m_2 \left( \frac{2}{3} \log\left(\frac{r}{R_\theta}\right) \vec{S}_1 \times \vec{a}_1 \cdot \vec{a}_2 - \frac{11}{18} \vec{S}_1 \times \vec{a}_1 \cdot \vec{a}_2 - \frac{11}{36} \vec{S}_1 \times \vec{v}_1 \cdot \vec{a}_2 - \frac{11}{36} \vec{S}_1 \times \vec{a}_1 \cdot \vec{a}_2 + \frac{2}{3} \hat{n} \times \vec{S}_1 \cdot \vec{a}_1 \hat{n} \cdot \vec{a}_2 + \right. \\ & \quad \frac{1}{3} \hat{n} \times \vec{S}_1 \cdot \vec{v}_1 \hat{n} \cdot \vec{a}_2 + \frac{1}{3} \hat{n} \times \vec{S}_1 \cdot \vec{a}_1 \hat{n} \cdot \vec{a}_2 + \frac{1}{3} \vec{S}_1 \times \vec{v}_1 \cdot \vec{a}_2 \log\left(\frac{r}{R_\theta}\right) + \\ & \quad \left. \frac{1}{3} \vec{S}_1 \times \vec{a}_1 \cdot \vec{a}_2 \log\left(\frac{r}{R_\theta}\right) + \frac{-\frac{1}{3} \vec{S}_1 \times \vec{a}_1 \cdot \vec{a}_2 - \frac{1}{6} \vec{S}_1 \times \vec{v}_1 \cdot \vec{a}_2 - \frac{1}{6} \vec{S}_1 \times \vec{a}_1 \cdot \vec{a}_2}{\epsilon_d} \right) G^2 \Big\} \end{aligned}$$

$$\left\{ \text{DiagSet}[2, 2, 96], \right.$$
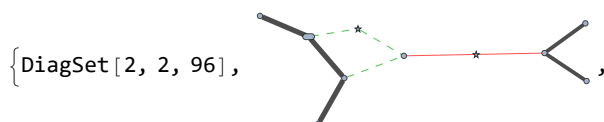

$$,$$

$$\begin{aligned} & \frac{1}{r} \left( \frac{4}{3} \hat{n} \times \vec{S}_1 \cdot \vec{a}_1 (\hat{n} \cdot \vec{v}_2)^2 + \frac{4}{3} \hat{n} \times \vec{S}_1 \cdot \vec{v}_1 (\hat{n} \cdot \vec{v}_2)^2 - \frac{4}{3} \vec{S}_1 \times \vec{a}_1 \cdot \vec{v}_2 \hat{n} \cdot \vec{v}_2 - 2 \vec{S}_1 \times \vec{v}_1 \cdot \vec{a}_1 \hat{n} \cdot \vec{v}_2 - \frac{4}{3} \vec{S}_1 \times \vec{v}_1 \cdot \vec{v}_2 \hat{n} \cdot \vec{v}_2 - \right. \\ & \quad \frac{4}{3} \vec{S}_1 \times \vec{v}_1 \cdot \vec{a}_1 \hat{n} \cdot \vec{v}_2 - \frac{1}{3} \hat{n} \times \vec{S}_1 \cdot \vec{v}_1 \hat{n} \cdot \vec{a}_1 \hat{n} \cdot \vec{v}_2 - \frac{4}{3} \hat{n} \times \vec{S}_1 \cdot \vec{v}_1 \hat{n} \cdot \vec{a}_1 \hat{n} \cdot \vec{v}_2 - \frac{1}{3} \hat{n} \times \vec{S}_1 \cdot \vec{a}_1 \hat{n} \cdot \vec{a}_1 \hat{n} \cdot \vec{v}_2 - \end{aligned}$$



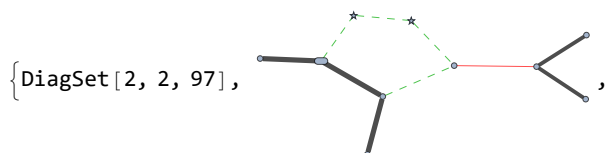

[illegible]

$$\begin{aligned}
& \left( \frac{15}{8} \hat{n} \times \vec{S}_1 \cdot \vec{v}_1 (\hat{n} \cdot \vec{v}_1)^4 + \vec{S}_1 \times \vec{v}_1 \cdot \vec{v}_2 (\hat{n} \cdot \vec{v}_1)^3 - 6 \hat{n} \times \vec{S}_1 \cdot \vec{v}_1 \hat{n} \cdot \vec{v}_2 (\hat{n} \cdot \vec{v}_1)^3 + 6 \hat{n} \times \vec{S}_1 \cdot \vec{v}_1 (\hat{n} \cdot \vec{v}_2)^2 (\hat{n} \cdot \vec{v}_1)^2 - \right. \\
& 2 \vec{S}_1 \times \vec{v}_1 \cdot \vec{v}_2 \hat{n} \cdot \vec{v}_2 (\hat{n} \cdot \vec{v}_1)^2 - \frac{21}{4} \hat{n} \times \vec{S}_1 \cdot \vec{v}_1 \vec{v}_1 \cdot \vec{v}_1 (\hat{n} \cdot \vec{v}_1)^2 + 3 \hat{n} \times \vec{S}_1 \cdot \vec{v}_1 \vec{v}_1 \cdot \vec{v}_2 (\hat{n} \cdot \vec{v}_1)^2 - \\
& \hat{n} \times \vec{S}_1 \cdot \vec{v}_1 \vec{v}_2 \cdot \vec{v}_2 (\hat{n} \cdot \vec{v}_1)^2 - 3 \vec{S}_1 \times \vec{v}_1 \cdot \vec{v}_2 \vec{v}_1 \cdot \vec{v}_1 \hat{n} \cdot \vec{v}_1 + 12 \hat{n} \times \vec{S}_1 \cdot \vec{v}_1 \hat{n} \cdot \vec{v}_2 \vec{v}_1 \cdot \vec{v}_1 \hat{n} \cdot \vec{v}_1 + \vec{S}_1 \times \vec{v}_1 \cdot \vec{v}_2 \vec{v}_1 \cdot \vec{v}_2 \hat{n} \cdot \vec{v}_1 - \\
& 4 \hat{n} \times \vec{S}_1 \cdot \vec{v}_1 \hat{n} \cdot \vec{v}_2 \vec{v}_1 \cdot \vec{v}_2 \hat{n} \cdot \vec{v}_1 + \frac{3}{8} \hat{n} \times \vec{S}_1 \cdot \vec{v}_1 (\vec{v}_1 \cdot \vec{v}_1)^2 + \frac{1}{2} \hat{n} \times \vec{S}_1 \cdot \vec{v}_1 (\vec{v}_1 \cdot \vec{v}_2)^2 - 10 \hat{n} \times \vec{S}_1 \cdot \vec{v}_1 (\hat{n} \cdot \vec{v}_2)^2 \vec{v}_1 \cdot \vec{v}_1 + \\
& 5 \vec{S}_1 \times \vec{v}_1 \cdot \vec{v}_2 \hat{n} \cdot \vec{v}_2 \vec{v}_1 \cdot \vec{v}_1 - 3 \hat{n} \times \vec{S}_1 \cdot \vec{v}_1 \vec{v}_1 \cdot \vec{v}_1 \vec{v}_1 \cdot \vec{v}_2 + \frac{5}{2} \hat{n} \times \vec{S}_1 \cdot \vec{v}_1 \vec{v}_1 \cdot \vec{v}_1 \vec{v}_2 \cdot \vec{v}_2 \Big) m_1 m_2 G^2 + \\
& r m_1 m_2 \left( \log \left( \frac{r}{R_\theta} \right) \hat{n} \times \vec{S}_1 \cdot \vec{a}_1 - \frac{\hat{n} \times \vec{S}_1 \cdot \vec{a}_1}{2 \epsilon_d} - \hat{n} \times \vec{S}_1 \cdot \vec{a}_1 \right) G^2 + \\
& m_1 m_2 \left( -\frac{8}{3} \log \left( \frac{r}{R_\theta} \right) \vec{S}_1 \times \vec{v}_1 \cdot \vec{a}_1 + \frac{19}{9} \vec{S}_1 \times \vec{v}_1 \cdot \vec{a}_1 + 2 \vec{S}_1 \times \vec{a}_1 \cdot \vec{v}_2 - \frac{1}{18} \vec{S}_1 \times \vec{v}_1 \cdot \vec{a}_1 + \right. \\
& \frac{2}{\vec{S}_1 \times \vec{v}_1 \cdot \vec{a}_2} + \frac{19}{18} \vec{S}_1 \times \vec{a}_1 \cdot \vec{a}_1 - \frac{1}{3} \hat{n} \times \vec{S}_1 \cdot \vec{v}_1 \hat{n} \cdot \vec{a}_1 - \frac{1}{6} \hat{n} \times \vec{S}_1 \cdot \vec{a}_1 \hat{n} \cdot \vec{a}_1 + \frac{5}{3} \hat{n} \times \vec{S}_1 \cdot \vec{v}_1 \hat{n} \cdot \vec{a}_1 - \\
& \frac{1}{3} \hat{n} \times \vec{S}_1 \cdot \vec{a}_1 \hat{n} \cdot \vec{a}_1 - \hat{n} \times \vec{S}_1 \cdot \vec{v}_1 \hat{n} \cdot \vec{a}_2 - \frac{2}{3} \hat{n} \times \vec{S}_1 \cdot \vec{a}_1 \hat{n} \cdot \vec{v}_1 + \frac{17}{6} \hat{n} \times \vec{S}_1 \cdot \vec{a}_1 \hat{n} \cdot \vec{v}_1 - \\
& 2 \hat{n} \times \vec{S}_1 \cdot \vec{a}_1 \hat{n} \cdot \vec{v}_2 - 2 \vec{S}_1 \times \vec{a}_1 \cdot \vec{v}_2 \log \left( \frac{r}{R_\theta} \right) + \frac{1}{3} \vec{S}_1 \times \vec{v}_1 \cdot \vec{a}_1 \log \left( \frac{r}{R_\theta} \right) - \vec{S}_1 \times \vec{v}_1 \cdot \vec{a}_2 \log \left( \frac{r}{R_\theta} \right) - \\
& \left. \frac{4}{3} \vec{S}_1 \times \vec{a}_1 \cdot \vec{a}_1 \log \left( \frac{r}{R_\theta} \right) + \frac{\frac{4}{3} \vec{S}_1 \times \vec{v}_1 \cdot \vec{a}_1 + \vec{S}_1 \times \vec{a}_1 \cdot \vec{v}_2 - \frac{1}{6} \vec{S}_1 \times \vec{v}_1 \cdot \vec{a}_1 + \frac{1}{2} \vec{S}_1 \times \vec{v}_1 \cdot \vec{a}_2 + \frac{2}{3} \vec{S}_1 \times \vec{a}_1 \cdot \vec{a}_1}{\epsilon_d} \right) G^2 \Big\}
\end{aligned}$$

$$\{ \text{DiagSet}[2, 2, 98], \text{Diagram}, \}$$
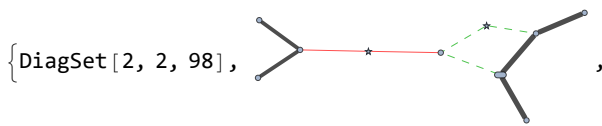

$$\begin{aligned}
& \frac{1}{r} \left( -\frac{4}{3} \hat{n} \times \vec{S}_1 \cdot \vec{a}_1 (\hat{n} \cdot \vec{v}_2)^2 - \frac{4}{3} \hat{n} \times \vec{S}_1 \cdot \vec{a}_1 (\hat{n} \cdot \vec{v}_2)^2 + \frac{4}{3} \vec{S}_1 \times \vec{a}_1 \cdot \vec{v}_2 \hat{n} \cdot \vec{v}_2 + \frac{2}{3} \vec{S}_1 \times \vec{v}_1 \cdot \vec{a}_1 \hat{n} \cdot \vec{v}_2 + \frac{4}{3} \vec{S}_1 \times \vec{a}_1 \cdot \vec{v}_2 \hat{n} \cdot \vec{v}_2 - \right. \\
& \hat{n} \times \vec{S}_1 \cdot \vec{v}_1 \hat{n} \cdot \vec{a}_1 \hat{n} \cdot \vec{v}_2 - \frac{2}{3} \hat{n} \times \vec{S}_1 \cdot \vec{v}_1 \hat{n} \cdot \vec{a}_1 \hat{n} \cdot \vec{v}_2 + \hat{n} \times \vec{S}_1 \cdot \vec{a}_1 \hat{n} \cdot \vec{a}_1 \hat{n} \cdot \vec{v}_2 + \frac{11}{3} \hat{n} \times \vec{S}_1 \cdot \vec{a}_1 \hat{n} \cdot \vec{v}_1 \hat{n} \cdot \vec{v}_2 + \\
& \frac{1}{3} \hat{n} \times \vec{S}_1 \cdot \vec{v}_1 \hat{n} \cdot \vec{v}_1 \hat{n} \cdot \vec{v}_2 + 2 \hat{n} \times \vec{S}_1 \cdot \vec{a}_1 \hat{n} \cdot \vec{v}_1 \hat{n} \cdot \vec{v}_2 + \frac{1}{2} \vec{S}_1 \times \vec{v}_1 \cdot \vec{v}_2 \hat{n} \cdot \vec{a}_1 + \frac{1}{3} \vec{S}_1 \times \vec{v}_1 \cdot \vec{v}_2 \hat{n} \cdot \vec{a}_1 - \\
& \frac{1}{2} \vec{S}_1 \times \vec{a}_1 \cdot \vec{v}_2 \hat{n} \cdot \vec{a}_1 - \frac{1}{6} \vec{S}_1 \times \vec{v}_1 \cdot \vec{a}_2 \hat{n} \cdot \vec{a}_1 + \frac{2}{3} \vec{S}_1 \times \vec{v}_1 \cdot \vec{a}_1 \hat{n} \cdot \vec{a}_2 + \frac{1}{3} \hat{n} \times \vec{S}_1 \cdot \vec{v}_1 \hat{n} \cdot \vec{a}_1 \hat{n} \cdot \vec{a}_2 - \\
& \frac{11}{6} \vec{S}_1 \times \vec{a}_1 \cdot \vec{v}_2 \hat{n} \cdot \vec{v}_1 - \frac{1}{6} \vec{S}_1 \times \vec{v}_1 \cdot \vec{a}_2 \hat{n} \cdot \vec{v}_1 - \frac{1}{6} \vec{S}_1 \times \vec{v}_1 \cdot \vec{v}_2 \hat{n} \cdot \vec{v}_1 - \vec{S}_1 \times \vec{a}_1 \cdot \vec{v}_2 \hat{n} \cdot \vec{v}_1 - \frac{5}{6} \vec{S}_1 \times \vec{a}_1 \cdot \vec{a}_2 \hat{n} \cdot \vec{v}_1 + \\
& \frac{1}{3} \hat{n} \times \vec{S}_1 \cdot \vec{v}_1 \hat{n} \cdot \vec{a}_2 \hat{n} \cdot \vec{v}_1 + \frac{5}{3} \hat{n} \times \vec{S}_1 \cdot \vec{a}_1 \hat{n} \cdot \vec{a}_2 \hat{n} \cdot \vec{v}_1 + \frac{1}{2} \hat{n} \times \vec{S}_1 \cdot \vec{v}_1 \vec{a}_1 \cdot \vec{v}_2 - \frac{1}{6} \hat{n} \times \vec{S}_1 \cdot \vec{v}_1 \vec{a}_1 \cdot \vec{a}_2 + \\
& \frac{1}{3} \hat{n} \times \vec{S}_1 \cdot \vec{v}_1 \vec{a}_1 \cdot \vec{v}_2 - \frac{1}{2} \hat{n} \times \vec{S}_1 \cdot \vec{a}_1 \vec{a}_1 \cdot \vec{v}_2 - \frac{1}{6} \hat{n} \times \vec{S}_1 \cdot \vec{v}_1 \vec{v}_1 \cdot \vec{a}_2 - \frac{5}{6} \hat{n} \times \vec{S}_1 \cdot \vec{a}_1 \vec{v}_1 \cdot \vec{a}_2 - \frac{11}{6} \hat{n} \times \vec{S}_1 \cdot \vec{a}_1 \vec{v}_1 \cdot \vec{v}_2 - \\
& \left. \frac{1}{6} \hat{n} \times \vec{S}_1 \cdot \vec{v}_1 \vec{v}_1 \cdot \vec{v}_2 - \hat{n} \times \vec{S}_1 \cdot \vec{a}_1 \vec{v}_1 \cdot \vec{v}_2 + \frac{2}{3} \hat{n} \times \vec{S}_1 \cdot \vec{a}_1 \vec{v}_2 \cdot \vec{v}_2 + \frac{2}{3} \hat{n} \times \vec{S}_1 \cdot \vec{a}_1 \vec{v}_2 \cdot \vec{v}_2 \right) m_1 m_2 G^2 + \frac{1}{r^2} \\
& \left( \frac{1}{2} \vec{S}_1 \times \vec{v}_1 \cdot \vec{v}_2 (\hat{n} \cdot \vec{v}_1)^2 + \frac{13}{6} \vec{S}_1 \times \vec{a}_1 \cdot \vec{v}_2 (\hat{n} \cdot \vec{v}_1)^2 + \frac{1}{3} \vec{S}_1 \times \vec{v}_1 \cdot \vec{a}_2 (\hat{n} \cdot \vec{v}_1)^2 - \frac{4}{3} \hat{n} \times \vec{S}_1 \cdot \vec{v}_1 \hat{n} \cdot \vec{a}_2 (\hat{n} \cdot \vec{v}_1)^2 - \right. \\
& 2 \hat{n} \times \vec{S}_1 \cdot \vec{v}_1 \hat{n} \cdot \vec{v}_2 (\hat{n} \cdot \vec{v}_1)^2 - \frac{26}{3} \hat{n} \times \vec{S}_1 \cdot \vec{a}_1 \hat{n} \cdot \vec{v}_2 (\hat{n} \cdot \vec{v}_1)^2 + \frac{4}{3} \hat{n} \times \vec{S}_1 \cdot \vec{v}_1 (\hat{n} \cdot \vec{v}_2)^2 \hat{n} \cdot \vec{v}_1 +
\end{aligned}$$

$$\begin{aligned}
& \frac{20}{3} \hat{n} \times \vec{S}_1 \cdot \vec{a}_1 (\hat{n} \cdot \vec{v}_2)^2 \hat{n} \cdot \vec{v}_1 - \frac{2}{3} \vec{S}_1 \times \vec{v}_1 \cdot \vec{v}_2 \hat{n} \cdot \vec{a}_1 \hat{n} \cdot \vec{v}_1 - \frac{2}{3} \vec{S}_1 \times \vec{v}_1 \cdot \vec{v}_2 \hat{n} \cdot \vec{v}_2 \hat{n} \cdot \vec{v}_1 - \\
& \frac{10}{3} \vec{S}_1 \times \vec{a}_1 \cdot \vec{v}_2 \hat{n} \cdot \vec{v}_2 \hat{n} \cdot \vec{v}_1 - 2 \vec{S}_1 \times \vec{v}_1 \cdot \vec{a}_1 \hat{n} \cdot \vec{v}_2 \hat{n} \cdot \vec{v}_1 + \frac{8}{3} \hat{n} \times \vec{S}_1 \cdot \vec{v}_1 \hat{n} \cdot \vec{a}_1 \hat{n} \cdot \vec{v}_2 \hat{n} \cdot \vec{v}_1 - \\
& \frac{2}{3} \hat{n} \times \vec{S}_1 \cdot \vec{v}_1 \vec{a}_1 \cdot \vec{v}_2 \hat{n} \cdot \vec{v}_1 + \frac{2}{3} \hat{n} \times \vec{S}_1 \cdot \vec{v}_1 \vec{v}_1 \cdot \vec{a}_2 \hat{n} \cdot \vec{v}_1 + \hat{n} \times \vec{S}_1 \cdot \vec{v}_1 \vec{v}_1 \cdot \vec{v}_2 \hat{n} \cdot \vec{v}_1 + \frac{13}{3} \hat{n} \times \vec{S}_1 \cdot \vec{a}_1 \vec{v}_1 \cdot \vec{v}_2 \hat{n} \cdot \vec{v}_1 - \\
& \frac{1}{3} \hat{n} \times \vec{S}_1 \cdot \vec{v}_1 \vec{v}_2 \cdot \vec{v}_2 \hat{n} \cdot \vec{v}_1 - \frac{5}{3} \hat{n} \times \vec{S}_1 \cdot \vec{a}_1 \vec{v}_2 \cdot \vec{v}_2 \hat{n} \cdot \vec{v}_1 + \frac{4}{3} \vec{S}_1 \times \vec{v}_1 \cdot \vec{a}_1 (\hat{n} \cdot \vec{v}_2)^2 + \frac{4}{3} \hat{n} \times \vec{S}_1 \cdot \vec{v}_1 \hat{n} \cdot \vec{a}_1 (\hat{n} \cdot \vec{v}_2)^2 - \\
& \frac{2}{3} \vec{S}_1 \times \vec{v}_1 \cdot \vec{v}_2 \hat{n} \cdot \vec{a}_1 \hat{n} \cdot \vec{v}_2 + \frac{1}{3} \vec{S}_1 \times \vec{v}_1 \cdot \vec{v}_2 \vec{a}_1 \cdot \vec{v}_2 - \frac{2}{3} \hat{n} \times \vec{S}_1 \cdot \vec{v}_1 \hat{n} \cdot \vec{v}_2 \vec{a}_1 \cdot \vec{v}_2 - \frac{1}{6} \vec{S}_1 \times \vec{v}_1 \cdot \vec{v}_2 \vec{v}_1 \cdot \vec{a}_1 + \\
& \frac{1}{3} \hat{n} \times \vec{S}_1 \cdot \vec{v}_1 \hat{n} \cdot \vec{v}_2 \vec{v}_1 \cdot \vec{a}_1 - \frac{1}{2} \vec{S}_1 \times \vec{v}_1 \cdot \vec{v}_2 \vec{v}_1 \cdot \vec{v}_1 - \frac{4}{3} \vec{S}_1 \times \vec{a}_1 \cdot \vec{v}_2 \vec{v}_1 \cdot \vec{v}_1 - \frac{1}{6} \vec{S}_1 \times \vec{v}_1 \cdot \vec{a}_2 \vec{v}_1 \cdot \vec{v}_1 + \\
& \frac{1}{3} \hat{n} \times \vec{S}_1 \cdot \vec{v}_1 \hat{n} \cdot \vec{a}_2 \vec{v}_1 \cdot \vec{v}_1 + \hat{n} \times \vec{S}_1 \cdot \vec{v}_1 \hat{n} \cdot \vec{v}_2 \vec{v}_1 \cdot \vec{v}_1 + \frac{8}{3} \hat{n} \times \vec{S}_1 \cdot \vec{a}_1 \hat{n} \cdot \vec{v}_2 \vec{v}_1 \cdot \vec{v}_1 + \frac{1}{3} \vec{S}_1 \times \vec{v}_1 \cdot \vec{v}_2 \vec{v}_1 \cdot \vec{v}_2 + \\
& \frac{5}{3} \vec{S}_1 \times \vec{a}_1 \cdot \vec{v}_2 \vec{v}_1 \cdot \vec{v}_2 + \vec{S}_1 \times \vec{v}_1 \cdot \vec{a}_1 \vec{v}_1 \cdot \vec{v}_2 - \frac{2}{3} \hat{n} \times \vec{S}_1 \cdot \vec{v}_1 \hat{n} \cdot \vec{a}_1 \vec{v}_1 \cdot \vec{v}_2 - \frac{2}{3} \hat{n} \times \vec{S}_1 \cdot \vec{v}_1 \hat{n} \cdot \vec{v}_2 \vec{v}_1 \cdot \vec{v}_2 - \\
& \frac{10}{3} \hat{n} \times \vec{S}_1 \cdot \vec{a}_1 \hat{n} \cdot \vec{v}_2 \vec{v}_1 \cdot \vec{v}_2 - \frac{2}{3} \vec{S}_1 \times \vec{v}_1 \cdot \vec{a}_1 \vec{v}_2 \cdot \vec{v}_2 - \frac{1}{3} \hat{n} \times \vec{S}_1 \cdot \vec{v}_1 \hat{n} \cdot \vec{a}_1 \vec{v}_2 \cdot \vec{v}_2 \Big) m_1 m_2 G^2 + \\
& \frac{1}{r^3} \left( -\frac{2}{3} \vec{S}_1 \times \vec{v}_1 \cdot \vec{v}_2 (\hat{n} \cdot \vec{v}_1)^3 + 4 \hat{n} \times \vec{S}_1 \cdot \vec{v}_1 \hat{n} \cdot \vec{v}_2 (\hat{n} \cdot \vec{v}_1)^3 - 8 \hat{n} \times \vec{S}_1 \cdot \vec{v}_1 (\hat{n} \cdot \vec{v}_2)^2 (\hat{n} \cdot \vec{v}_1)^2 + \right. \\
& \frac{8}{3} \vec{S}_1 \times \vec{v}_1 \cdot \vec{v}_2 \hat{n} \cdot \vec{v}_2 (\hat{n} \cdot \vec{v}_1)^2 - 2 \hat{n} \times \vec{S}_1 \cdot \vec{v}_1 \vec{v}_1 \cdot \vec{v}_2 (\hat{n} \cdot \vec{v}_1)^2 + \frac{4}{3} \hat{n} \times \vec{S}_1 \cdot \vec{v}_1 \vec{v}_2 \cdot \vec{v}_2 (\hat{n} \cdot \vec{v}_1)^2 + \\
& \vec{S}_1 \times \vec{v}_1 \cdot \vec{v}_2 \vec{v}_1 \cdot \vec{v}_1 \hat{n} \cdot \vec{v}_1 - 4 \hat{n} \times \vec{S}_1 \cdot \vec{v}_1 \hat{n} \cdot \vec{v}_2 \vec{v}_1 \cdot \vec{v}_1 \hat{n} \cdot \vec{v}_1 - \frac{4}{3} \vec{S}_1 \times \vec{v}_1 \cdot \vec{v}_2 \vec{v}_1 \cdot \vec{v}_2 \hat{n} \cdot \vec{v}_1 + \\
& \frac{16}{3} \hat{n} \times \vec{S}_1 \cdot \vec{v}_1 \hat{n} \cdot \vec{v}_2 \vec{v}_1 \cdot \vec{v}_2 \hat{n} \cdot \vec{v}_1 - \frac{2}{3} \hat{n} \times \vec{S}_1 \cdot \vec{v}_1 (\vec{v}_1 \cdot \vec{v}_2)^2 + \frac{4}{3} \hat{n} \times \vec{S}_1 \cdot \vec{v}_1 (\hat{n} \cdot \vec{v}_2)^2 \vec{v}_1 \cdot \vec{v}_1 - \\
& \left. \frac{2}{3} \vec{S}_1 \times \vec{v}_1 \cdot \vec{v}_2 \hat{n} \cdot \vec{v}_2 \vec{v}_1 \cdot \vec{v}_1 + \hat{n} \times \vec{S}_1 \cdot \vec{v}_1 \vec{v}_1 \cdot \vec{v}_1 \vec{v}_1 \cdot \vec{v}_2 - \frac{1}{3} \hat{n} \times \vec{S}_1 \cdot \vec{v}_1 \vec{v}_1 \cdot \vec{v}_1 \vec{v}_2 \cdot \vec{v}_2 \right) m_1 m_2 G^2 + \\
& m_1 m_2 \left( -\frac{2}{3} \log\left(\frac{r}{R_\theta}\right) \vec{S}_1 \times \vec{a}_1 \cdot \vec{v}_2 + \frac{7}{9} \vec{S}_1 \times \vec{a}_1 \cdot \vec{v}_2 + \frac{7}{9} \vec{S}_1 \times \vec{a}_1 \cdot \vec{a}_2 + \frac{7}{9} \vec{S}_1 \times \vec{a}_1 \cdot \vec{v}_2 + \frac{7}{9} \vec{S}_1 \times \vec{a}_1 \cdot \vec{a}_2 - \right. \\
& \frac{2}{3} \hat{n} \times \vec{S}_1 \cdot \vec{a}_1 \hat{n} \cdot \vec{a}_2 - \frac{2}{3} \hat{n} \times \vec{S}_1 \cdot \vec{a}_1 \hat{n} \cdot \vec{a}_2 - \frac{2}{3} \hat{n} \times \vec{S}_1 \cdot \vec{a}_1 \hat{n} \cdot \vec{v}_2 - \frac{2}{3} \hat{n} \times \vec{S}_1 \cdot \vec{a}_1 \hat{n} \cdot \vec{v}_2 - \frac{2}{3} \vec{S}_1 \times \vec{a}_1 \cdot \vec{a}_2 \log\left(\frac{r}{R_\theta}\right) - \\
& \left. \frac{2}{3} \vec{S}_1 \times \vec{a}_1 \cdot \vec{v}_2 \log\left(\frac{r}{R_\theta}\right) - \frac{2}{3} \vec{S}_1 \times \vec{a}_1 \cdot \vec{a}_2 \log\left(\frac{r}{R_\theta}\right) + \frac{\frac{1}{3} \vec{S}_1 \times \vec{a}_1 \cdot \vec{v}_2 + \frac{1}{3} \vec{S}_1 \times \vec{a}_1 \cdot \vec{a}_2 + \frac{1}{3} \vec{S}_1 \times \vec{a}_1 \cdot \vec{v}_2 + \frac{1}{3} \vec{S}_1 \times \vec{a}_1 \cdot \vec{a}_2}{\epsilon_d} \right) G^2 \Big\}
\end{aligned}$$

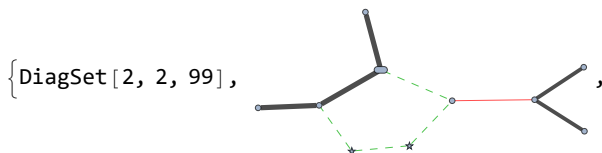

$$\begin{aligned}
& \frac{1}{r} \left( \frac{3}{4} \hat{n} \times \vec{S}_1 \cdot \vec{v}_1 (\hat{n} \cdot \vec{a}_1)^2 + \frac{2}{3} \vec{S}_1 \times \vec{v}_1 \cdot \vec{v}_2 \hat{n} \cdot \vec{a}_1 + \frac{1}{3} \vec{S}_1 \times \vec{v}_1 \cdot \vec{a}_2 \hat{n} \cdot \vec{a}_1 - \frac{2}{3} \hat{n} \times \vec{S}_1 \cdot \vec{v}_1 \hat{n} \cdot \vec{a}_2 \hat{n} \cdot \vec{a}_1 + 3 \hat{n} \times \vec{S}_1 \cdot \vec{v}_1 \hat{n} \cdot \vec{v}_1 \hat{n} \cdot \vec{a}_1 - \right. \\
& \frac{3}{2} \hat{n} \times \vec{S}_1 \cdot \vec{a}_1 \hat{n} \cdot \vec{v}_1 \hat{n} \cdot \vec{a}_1 - \frac{4}{3} \hat{n} \times \vec{S}_1 \cdot \vec{v}_1 \hat{n} \cdot \vec{v}_2 \hat{n} \cdot \vec{a}_1 - \frac{9}{2} \hat{n} \times \vec{S}_1 \cdot \vec{a}_1 (\hat{n} \cdot \vec{v}_1)^2 - \frac{1}{12} \hat{n} \times \vec{S}_1 \cdot \vec{v}_1 (\hat{n} \cdot \vec{v}_1)^2 + \\
& \frac{15}{4} \hat{n} \times \vec{S}_1 \cdot \vec{a}_1 (\hat{n} \cdot \vec{v}_1)^2 + \frac{2}{3} \hat{n} \times \vec{S}_1 \cdot \vec{a}_1 (\hat{n} \cdot \vec{v}_2)^2 - \vec{S}_1 \times \vec{v}_1 \cdot \vec{v}_2 \hat{n} \cdot \vec{a}_1 - \frac{1}{3} \vec{S}_1 \times \vec{v}_1 \cdot \vec{a}_1 \hat{n} \cdot \vec{a}_2 - \frac{5}{3} \vec{S}_1 \times \vec{a}_1 \cdot \vec{v}_2 \hat{n} \cdot \vec{v}_1 - \\
& \left. \frac{1}{3} \vec{S}_1 \times \vec{v}_1 \cdot \vec{a}_1 \hat{n} \cdot \vec{v}_1 + 2 \vec{S}_1 \times \vec{a}_1 \cdot \vec{v}_2 \hat{n} \cdot \vec{v}_1 - \frac{5}{6} \vec{S}_1 \times \vec{a}_1 \cdot \vec{a}_2 \hat{n} \cdot \vec{v}_1 + 2 \vec{S}_1 \times \vec{v}_1 \cdot \vec{a}_1 \hat{n} \cdot \vec{v}_1 - \frac{5}{2} \hat{n} \times \vec{S}_1 \cdot \vec{v}_1 \hat{n} \cdot \vec{a}_1 \hat{n} \cdot \vec{v}_1 + \right.
\end{aligned}$$

$$\begin{aligned}
& \frac{5}{3} \hat{n} \times \vec{S}_1 \cdot \vec{a}_1 \hat{n} \cdot \vec{a}_2 \hat{n} \cdot \vec{v}_1 - \frac{2}{3} \vec{S}_1 \times \vec{v}_1 \cdot \vec{a}_1 \hat{n} \cdot \vec{v}_2 - \frac{2}{3} \vec{S}_1 \times \vec{a}_1 \cdot \vec{v}_2 \hat{n} \cdot \vec{v}_2 + 2 \hat{n} \times \vec{S}_1 \cdot \vec{v}_1 \hat{n} \cdot \vec{a}_1 \hat{n} \cdot \vec{v}_2 + \\
& \frac{10}{3} \hat{n} \times \vec{S}_1 \cdot \vec{a}_1 \hat{n} \cdot \vec{v}_1 \hat{n} \cdot \vec{v}_2 - 4 \hat{n} \times \vec{S}_1 \cdot \vec{a}_1 \hat{n} \cdot \vec{v}_1 \hat{n} \cdot \vec{v}_2 - \hat{n} \times \vec{S}_1 \cdot \vec{v}_1 \vec{a}_1 \cdot \vec{v}_2 - \frac{3}{4} \hat{n} \times \vec{S}_1 \cdot \vec{v}_1 \vec{a}_1 \cdot \vec{a}_1 + \frac{1}{3} \hat{n} \times \vec{S}_1 \cdot \vec{v}_1 \vec{a}_1 \cdot \vec{a}_2 + \\
& \frac{2}{3} \hat{n} \times \vec{S}_1 \cdot \vec{v}_1 \vec{a}_1 \cdot \vec{v}_2 + \frac{1}{2} \hat{n} \times \vec{S}_1 \cdot \vec{v}_1 \vec{v}_1 \cdot \vec{a}_1 - \frac{5}{6} \hat{n} \times \vec{S}_1 \cdot \vec{a}_1 \vec{v}_1 \cdot \vec{a}_2 - \frac{3}{2} \hat{n} \times \vec{S}_1 \cdot \vec{a}_1 \vec{v}_1 \cdot \vec{v}_1 + \frac{5}{12} \hat{n} \times \vec{S}_1 \cdot \vec{v}_1 \vec{v}_1 \cdot \vec{v}_1 - \\
& \frac{3}{4} \hat{n} \times \vec{S}_1 \cdot \vec{a}_1 \vec{v}_1 \cdot \vec{v}_1 - \frac{5}{3} \hat{n} \times \vec{S}_1 \cdot \vec{a}_1 \vec{v}_1 \cdot \vec{v}_2 + 2 \hat{n} \times \vec{S}_1 \cdot \vec{a}_1 \vec{v}_1 \cdot \vec{v}_2 - \frac{1}{3} \hat{n} \times \vec{S}_1 \cdot \vec{a}_1 \vec{v}_2 \cdot \vec{v}_2 \Big) m_1 m_2 G^2 + \frac{1}{r^2} \\
& \left( \frac{1}{3} \hat{n} \times \vec{S}_1 \cdot \vec{v}_1 (\hat{n} \cdot \vec{v}_1)^3 + \frac{32}{3} \hat{n} \times \vec{S}_1 \cdot \vec{a}_1 (\hat{n} \cdot \vec{v}_1)^3 + \frac{1}{6} \vec{S}_1 \times \vec{v}_1 \cdot \vec{v}_2 (\hat{n} \cdot \vec{v}_1)^2 + \frac{9}{2} \vec{S}_1 \times \vec{a}_1 \cdot \vec{v}_2 (\hat{n} \cdot \vec{v}_1)^2 + \right. \\
& \frac{25}{4} \vec{S}_1 \times \vec{v}_1 \cdot \vec{a}_1 (\hat{n} \cdot \vec{v}_1)^2 + \frac{1}{12} \vec{S}_1 \times \vec{v}_1 \cdot \vec{a}_2 (\hat{n} \cdot \vec{v}_1)^2 - 8 \hat{n} \times \vec{S}_1 \cdot \vec{v}_1 \hat{n} \cdot \vec{a}_1 (\hat{n} \cdot \vec{v}_1)^2 - \frac{1}{3} \hat{n} \times \vec{S}_1 \cdot \vec{v}_1 \hat{n} \cdot \vec{a}_2 (\hat{n} \cdot \vec{v}_1)^2 - \\
& \frac{2}{3} \hat{n} \times \vec{S}_1 \cdot \vec{v}_1 \hat{n} \cdot \vec{v}_2 (\hat{n} \cdot \vec{v}_1)^2 - 18 \hat{n} \times \vec{S}_1 \cdot \vec{a}_1 \hat{n} \cdot \vec{v}_2 (\hat{n} \cdot \vec{v}_1)^2 + \frac{20}{3} \hat{n} \times \vec{S}_1 \cdot \vec{a}_1 (\hat{n} \cdot \vec{v}_2)^2 \hat{n} \cdot \vec{v}_1 - \\
& 3 \vec{S}_1 \times \vec{v}_1 \cdot \vec{v}_2 \hat{n} \cdot \vec{a}_1 \hat{n} \cdot \vec{v}_1 - \frac{10}{3} \vec{S}_1 \times \vec{a}_1 \cdot \vec{v}_2 \hat{n} \cdot \vec{v}_2 \hat{n} \cdot \vec{v}_1 - 6 \vec{S}_1 \times \vec{v}_1 \cdot \vec{a}_1 \hat{n} \cdot \vec{v}_2 \hat{n} \cdot \vec{v}_1 + 12 \hat{n} \times \vec{S}_1 \cdot \vec{v}_1 \hat{n} \cdot \vec{a}_1 \hat{n} \cdot \vec{v}_2 \hat{n} \cdot \vec{v}_1 - \\
& 3 \hat{n} \times \vec{S}_1 \cdot \vec{v}_1 \vec{a}_1 \cdot \vec{v}_2 \hat{n} \cdot \vec{v}_1 + \frac{5}{2} \hat{n} \times \vec{S}_1 \cdot \vec{v}_1 \vec{v}_1 \cdot \vec{a}_1 \hat{n} \cdot \vec{v}_1 + \frac{1}{6} \hat{n} \times \vec{S}_1 \cdot \vec{v}_1 \vec{v}_1 \cdot \vec{a}_2 \hat{n} \cdot \vec{v}_1 - \hat{n} \times \vec{S}_1 \cdot \vec{v}_1 \vec{v}_1 \cdot \vec{v}_1 \hat{n} \cdot \vec{v}_1 + \\
& \hat{n} \times \vec{S}_1 \cdot \vec{a}_1 \vec{v}_1 \cdot \vec{v}_1 \hat{n} \cdot \vec{v}_1 + \frac{1}{3} \hat{n} \times \vec{S}_1 \cdot \vec{v}_1 \vec{v}_1 \cdot \vec{v}_2 \hat{n} \cdot \vec{v}_1 + 9 \hat{n} \times \vec{S}_1 \cdot \vec{a}_1 \vec{v}_1 \cdot \vec{v}_2 \hat{n} \cdot \vec{v}_1 - \frac{5}{3} \hat{n} \times \vec{S}_1 \cdot \vec{a}_1 \vec{v}_2 \cdot \vec{v}_2 \hat{n} \cdot \vec{v}_1 - \\
& \frac{2}{3} \vec{S}_1 \times \vec{v}_1 \cdot \vec{a}_1 (\hat{n} \cdot \vec{v}_2)^2 - \frac{8}{3} \hat{n} \times \vec{S}_1 \cdot \vec{v}_1 \hat{n} \cdot \vec{a}_1 (\hat{n} \cdot \vec{v}_2)^2 + \frac{4}{3} \vec{S}_1 \times \vec{v}_1 \cdot \vec{v}_2 \hat{n} \cdot \vec{a}_1 \hat{n} \cdot \vec{v}_2 - \frac{2}{3} \vec{S}_1 \times \vec{v}_1 \cdot \vec{v}_2 \vec{a}_1 \cdot \vec{v}_2 + \\
& \frac{4}{3} \hat{n} \times \vec{S}_1 \cdot \vec{v}_1 \hat{n} \cdot \vec{v}_2 \vec{a}_1 \cdot \vec{v}_2 - \frac{5}{6} \vec{S}_1 \times \vec{v}_1 \cdot \vec{v}_2 \vec{v}_1 \cdot \vec{v}_1 + \frac{3}{2} \vec{S}_1 \times \vec{a}_1 \cdot \vec{v}_2 \vec{v}_1 \cdot \vec{v}_1 + \frac{7}{4} \vec{S}_1 \times \vec{v}_1 \cdot \vec{a}_1 \vec{v}_1 \cdot \vec{v}_1 - \\
& \frac{5}{12} \vec{S}_1 \times \vec{v}_1 \cdot \vec{a}_2 \vec{v}_1 \cdot \vec{v}_1 - \frac{5}{2} \hat{n} \times \vec{S}_1 \cdot \vec{v}_1 \hat{n} \cdot \vec{a}_1 \vec{v}_1 \cdot \vec{v}_1 + \frac{5}{6} \hat{n} \times \vec{S}_1 \cdot \vec{v}_1 \hat{n} \cdot \vec{a}_2 \vec{v}_1 \cdot \vec{v}_1 + \frac{5}{3} \hat{n} \times \vec{S}_1 \cdot \vec{v}_1 \hat{n} \cdot \vec{v}_2 \vec{v}_1 \cdot \vec{v}_1 - \\
& 3 \hat{n} \times \vec{S}_1 \cdot \vec{a}_1 \hat{n} \cdot \vec{v}_2 \vec{v}_1 \cdot \vec{v}_1 + \frac{5}{3} \vec{S}_1 \times \vec{a}_1 \cdot \vec{v}_2 \vec{v}_1 \cdot \vec{v}_2 + 3 \vec{S}_1 \times \vec{v}_1 \cdot \vec{a}_1 \vec{v}_1 \cdot \vec{v}_2 - 3 \hat{n} \times \vec{S}_1 \cdot \vec{v}_1 \hat{n} \cdot \vec{a}_1 \vec{v}_1 \cdot \vec{v}_2 - \\
& \frac{10}{3} \hat{n} \times \vec{S}_1 \cdot \vec{a}_1 \hat{n} \cdot \vec{v}_2 \vec{v}_1 \cdot \vec{v}_2 + \frac{1}{3} \vec{S}_1 \times \vec{v}_1 \cdot \vec{a}_1 \vec{v}_2 \cdot \vec{v}_2 + \frac{2}{3} \hat{n} \times \vec{S}_1 \cdot \vec{v}_1 \hat{n} \cdot \vec{a}_1 \vec{v}_2 \cdot \vec{v}_2 \Big) m_1 m_2 G^2 + \frac{1}{r^3} \\
& \left( -\frac{5}{8} \hat{n} \times \vec{S}_1 \cdot \vec{v}_1 (\hat{n} \cdot \vec{v}_1)^4 - \frac{1}{3} \vec{S}_1 \times \vec{v}_1 \cdot \vec{v}_2 (\hat{n} \cdot \vec{v}_1)^3 + 2 \hat{n} \times \vec{S}_1 \cdot \vec{v}_1 \hat{n} \cdot \vec{v}_2 (\hat{n} \cdot \vec{v}_1)^3 - 2 \hat{n} \times \vec{S}_1 \cdot \vec{v}_1 (\hat{n} \cdot \vec{v}_2)^2 (\hat{n} \cdot \vec{v}_1)^2 + \right. \\
& \frac{2}{3} \vec{S}_1 \times \vec{v}_1 \cdot \vec{v}_2 \hat{n} \cdot \vec{v}_2 (\hat{n} \cdot \vec{v}_1)^2 + \frac{7}{4} \hat{n} \times \vec{S}_1 \cdot \vec{v}_1 \vec{v}_1 \cdot \vec{v}_1 (\hat{n} \cdot \vec{v}_1)^2 - \hat{n} \times \vec{S}_1 \cdot \vec{v}_1 \vec{v}_1 \cdot \vec{v}_2 (\hat{n} \cdot \vec{v}_1)^2 + \\
& \frac{1}{3} \hat{n} \times \vec{S}_1 \cdot \vec{v}_1 \vec{v}_2 \cdot \vec{v}_2 (\hat{n} \cdot \vec{v}_1)^2 + \vec{S}_1 \times \vec{v}_1 \cdot \vec{v}_2 \vec{v}_1 \cdot \vec{v}_1 \hat{n} \cdot \vec{v}_1 - 4 \hat{n} \times \vec{S}_1 \cdot \vec{v}_1 \hat{n} \cdot \vec{v}_2 \vec{v}_1 \cdot \vec{v}_1 \hat{n} \cdot \vec{v}_1 - \frac{1}{3} \vec{S}_1 \times \vec{v}_1 \cdot \vec{v}_2 \vec{v}_1 \cdot \vec{v}_2 \hat{n} \cdot \vec{v}_1 + \\
& \frac{4}{3} \hat{n} \times \vec{S}_1 \cdot \vec{v}_1 \hat{n} \cdot \vec{v}_2 \vec{v}_1 \cdot \vec{v}_2 \hat{n} \cdot \vec{v}_1 - \frac{1}{8} \hat{n} \times \vec{S}_1 \cdot \vec{v}_1 (\vec{v}_1 \cdot \vec{v}_1)^2 - \frac{1}{6} \hat{n} \times \vec{S}_1 \cdot \vec{v}_1 (\vec{v}_1 \cdot \vec{v}_2)^2 + \frac{10}{3} \hat{n} \times \vec{S}_1 \cdot \vec{v}_1 (\hat{n} \cdot \vec{v}_2)^2 \vec{v}_1 \cdot \vec{v}_1 - \\
& \frac{5}{3} \vec{S}_1 \times \vec{v}_1 \cdot \vec{v}_2 \hat{n} \cdot \vec{v}_2 \vec{v}_1 \cdot \vec{v}_1 + \hat{n} \times \vec{S}_1 \cdot \vec{v}_1 \vec{v}_1 \cdot \vec{v}_1 \vec{v}_1 \cdot \vec{v}_2 - \frac{5}{6} \hat{n} \times \vec{S}_1 \cdot \vec{v}_1 \vec{v}_1 \cdot \vec{v}_1 \vec{v}_2 \cdot \vec{v}_2 \Big) m_1 m_2 G^2 + \\
& r m_1 m_2 \left( -\frac{1}{3} \log \left( \frac{r}{R_\theta} \right) \hat{n} \times \vec{S}_1 \cdot \vec{a}_1 + \frac{\hat{n} \times \vec{S}_1 \cdot \vec{a}_1}{6 \in_d} + \frac{5}{9} \hat{n} \times \vec{S}_1 \cdot \vec{a}_1 \right) G^2 + \\
& m_1 m_2 \left( \frac{2}{3} \log \left( \frac{r}{R_\theta} \right) \frac{1}{\vec{S}_1 \times \vec{a}_1 \cdot \vec{v}_2} - \frac{10}{9} \frac{1}{\vec{S}_1 \times \vec{a}_1 \cdot \vec{v}_2} - \frac{1}{\vec{S}_1 \times \vec{v}_1 \cdot \vec{a}_1} - \frac{1}{18} \frac{2}{\vec{S}_1 \times \vec{v}_1 \cdot \vec{a}_1} - \frac{5}{9} \frac{1}{\vec{S}_1 \times \vec{a}_1 \cdot \vec{a}_2} - \right. \\
& \frac{1}{2} \vec{S}_1 \times \vec{a}_1 \cdot \vec{a}_1 + \hat{n} \times \vec{S}_1 \cdot \vec{v}_1 \hat{n} \cdot \vec{a}_1 + \frac{1}{2} \hat{n} \times \vec{S}_1 \cdot \vec{a}_1 \hat{n} \cdot \vec{a}_1 - \frac{1}{3} \hat{n} \times \vec{S}_1 \cdot \vec{v}_1 \hat{n} \cdot \vec{a}_1 - \hat{n} \times \vec{S}_1 \cdot \vec{a}_1 \hat{n} \cdot \vec{a}_1 + \\
& \left. \frac{1}{3} \hat{n} \times \vec{S}_1 \cdot \vec{a}_1 \hat{n} \cdot \vec{a}_2 - 2 \hat{n} \times \vec{S}_1 \cdot \vec{a}_1 \hat{n} \cdot \vec{v}_1 + \frac{5}{6} \hat{n} \times \vec{S}_1 \cdot \vec{a}_1 \hat{n} \cdot \vec{v}_1 + \frac{2}{3} \hat{n} \times \vec{S}_1 \cdot \vec{a}_1 \hat{n} \cdot \vec{v}_2 + \right.
\end{aligned}$$



$$\left. \frac{1}{3} \frac{\vec{S}_1 \times \vec{v}_1 \cdot \vec{a}_1}{S_1} \log\left(\frac{r}{R_\theta}\right) + \frac{1}{3} \frac{\vec{S}_1 \times \vec{a}_1 \cdot \vec{a}_2}{S_1} \log\left(\frac{r}{R_\theta}\right) + \frac{-\frac{1}{3} \frac{\vec{S}_1 \times \vec{a}_1 \cdot \vec{v}_2}{S_1} - \frac{1}{6} \frac{\vec{S}_1 \times \vec{v}_1 \cdot \vec{a}_1}{S_1} - \frac{1}{6} \frac{\vec{S}_1 \times \vec{a}_1 \cdot \vec{a}_2}{S_1}}{\epsilon_d} \right\} G^2$$

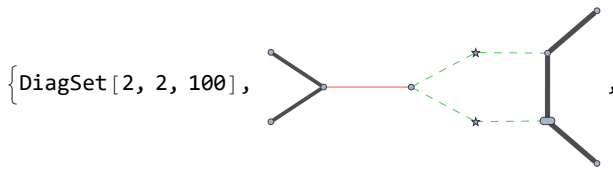

[illegible]

$$\begin{aligned}
& \frac{2}{3} \hat{n} \times \vec{S}_1 \cdot \vec{v}_1 \vec{v}_2 \cdot \vec{v}_2 (\hat{n} \cdot \vec{v}_1)^2 + \frac{2}{3} \vec{S}_1 \times \vec{v}_1 \cdot \vec{v}_2 \vec{v}_1 \cdot \vec{v}_2 \hat{n} \cdot \vec{v}_1 - \frac{8}{3} \hat{n} \times \vec{S}_1 \cdot \vec{v}_1 \hat{n} \cdot \vec{v}_2 \vec{v}_1 \cdot \vec{v}_2 \hat{n} \cdot \vec{v}_1 - \frac{1}{4} \hat{n} \times \vec{S}_1 \cdot \vec{v}_1 (\vec{v}_1 \cdot \vec{v}_1)^2 + \\
& \frac{1}{3} \hat{n} \times \vec{S}_1 \cdot \vec{v}_1 (\vec{v}_1 \cdot \vec{v}_2)^2 + \frac{4}{3} \hat{n} \times \vec{S}_1 \cdot \vec{v}_1 (\hat{n} \cdot \vec{v}_2)^2 \vec{v}_1 \cdot \vec{v}_1 - \frac{2}{3} \vec{S}_1 \times \vec{v}_1 \cdot \vec{v}_2 \hat{n} \cdot \vec{v}_2 \vec{v}_1 \cdot \vec{v}_1 - \frac{1}{3} \hat{n} \times \vec{S}_1 \cdot \vec{v}_1 \vec{v}_1 \cdot \vec{v}_1 \vec{v}_2 \cdot \vec{v}_2 \Big) \\
& m_1 m_2 G^2 + r m_1 m_2 \left( -\frac{2}{3} \log\left(\frac{r}{R_\theta}\right) \hat{n} \times \vec{S}_1 \cdot \frac{1}{\vec{a}_1} + \frac{\hat{n} \times \vec{S}_1 \cdot \frac{1}{\vec{a}_1}}{3 \in_d} - \frac{2}{9} \hat{n} \times \vec{S}_1 \cdot \frac{1}{\vec{a}_1} \right) G^2 + \\
& m_1 m_2 \left( \frac{2}{3} \log\left(\frac{r}{R_\theta}\right) \frac{1}{\vec{S}_1 \times \vec{a}_1} \cdot \vec{v}_2 + \frac{2}{9} \frac{1}{\vec{S}_1 \times \vec{a}_1} \cdot \vec{v}_2 + \frac{2}{9} \frac{1}{\vec{S}_1 \times \vec{a}_1} \cdot \vec{a}_2 + \frac{22}{9} \frac{1}{\vec{S}_1 \times \vec{v}_1} \cdot \frac{1}{\vec{a}_1} + \frac{2}{9} \frac{2}{\vec{S}_1 \times \vec{a}_1} \cdot \vec{v}_2 - \right. \\
& \frac{2}{\vec{S}_1 \times \vec{v}_1} \cdot \vec{a}_1 + \frac{11}{9} \vec{S}_1 \times \vec{a}_1 \cdot \frac{1}{\vec{a}_1} - \frac{2}{3} \hat{n} \times \vec{S}_1 \cdot \vec{v}_1 \hat{n} \cdot \frac{1}{\vec{a}_1} - \frac{1}{3} \hat{n} \times \vec{S}_1 \cdot \vec{a}_1 \hat{n} \cdot \frac{1}{\vec{a}_1} + \frac{2}{3} \hat{n} \times \vec{S}_1 \cdot \vec{a}_1 \hat{n} \cdot \vec{a}_2 - \\
& \hat{n} \times \vec{S}_1 \cdot \vec{a}_1 \hat{n} \cdot \vec{v}_1 + \frac{2}{3} \hat{n} \times \vec{S}_1 \cdot \frac{1}{\vec{a}_1} \hat{n} \cdot \vec{v}_2 + \frac{2}{3} \hat{n} \times \vec{S}_1 \cdot \vec{a}_1 \hat{n} \cdot \vec{v}_2 + \frac{2}{3} \frac{1}{\vec{S}_1 \times \vec{a}_1} \cdot \vec{a}_2 \log\left(\frac{r}{R_\theta}\right) - \\
& \frac{8}{3} \frac{1}{\vec{S}_1 \times \vec{v}_1} \cdot \frac{1}{\vec{a}_1} \log\left(\frac{r}{R_\theta}\right) + \frac{2}{3} \frac{2}{\vec{S}_1 \times \vec{a}_1} \cdot \vec{v}_2 \log\left(\frac{r}{R_\theta}\right) + 2 \vec{S}_1 \times \vec{v}_1 \cdot \vec{a}_1 \log\left(\frac{r}{R_\theta}\right) - \frac{4}{3} \vec{S}_1 \times \vec{a}_1 \cdot \frac{1}{\vec{a}_1} \log\left(\frac{r}{R_\theta}\right) + \\
& \left. \frac{1}{\in_d} \left( -\frac{1}{3} \frac{1}{\vec{S}_1 \times \vec{a}_1} \cdot \vec{v}_2 - \frac{1}{3} \frac{1}{\vec{S}_1 \times \vec{a}_1} \cdot \vec{a}_2 + \frac{4}{3} \frac{1}{\vec{S}_1 \times \vec{v}_1} \cdot \frac{1}{\vec{a}_1} - \frac{1}{3} \frac{2}{\vec{S}_1 \times \vec{a}_1} \cdot \vec{v}_2 - \frac{2}{\vec{S}_1 \times \vec{v}_1} \cdot \vec{a}_1 + \frac{2}{3} \vec{S}_1 \times \vec{a}_1 \cdot \frac{1}{\vec{a}_1} \right) \right) G^2 \Big\}
\end{aligned}$$

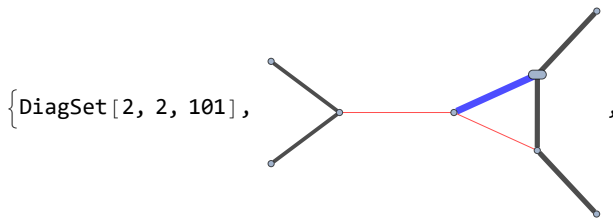

$$\begin{aligned}
& \frac{1}{r^2} \left( -3 \vec{S}_1 \times \vec{v}_1 \cdot \vec{a}_1 (\hat{n} \cdot \vec{v}_1)^2 + 4 \vec{S}_1 \times \vec{v}_1 \cdot \vec{a}_1 \hat{n} \cdot \vec{v}_2 \hat{n} \cdot \vec{v}_1 + 7 \hat{n} \times \vec{S}_1 \cdot \vec{v}_1 \vec{v}_1 \cdot \vec{a}_1 \hat{n} \cdot \vec{v}_1 + \right. \\
& \frac{25}{2} \hat{n} \times \vec{S}_1 \cdot \vec{v}_1 \vec{v}_1 \cdot \vec{v}_1 \hat{n} \cdot \vec{v}_1 + 17 \hat{n} \times \vec{S}_1 \cdot \vec{a}_1 \vec{v}_1 \cdot \vec{v}_1 \hat{n} \cdot \vec{v}_1 + 3 \hat{n} \times \vec{S}_1 \cdot \vec{v}_1 \vec{v}_2 \cdot \vec{a}_2 \hat{n} \cdot \vec{v}_1 + 9 \hat{n} \times \vec{S}_1 \cdot \vec{v}_1 \vec{v}_2 \cdot \vec{v}_2 \hat{n} \cdot \vec{v}_1 + \\
& 12 \hat{n} \times \vec{S}_1 \cdot \vec{a}_1 \vec{v}_2 \cdot \vec{v}_2 \hat{n} \cdot \vec{v}_1 + 6 \vec{S}_1 \times \vec{v}_1 \cdot \vec{v}_2 \vec{v}_1 \cdot \vec{a}_1 - 12 \hat{n} \times \vec{S}_1 \cdot \vec{v}_1 \hat{n} \cdot \vec{v}_2 \vec{v}_1 \cdot \vec{a}_1 + 6 \vec{S}_1 \times \vec{v}_1 \cdot \vec{a}_1 \vec{v}_1 \cdot \vec{v}_1 + \\
& 8 \hat{n} \times \vec{S}_1 \cdot \vec{v}_1 \hat{n} \cdot \vec{a}_1 \vec{v}_1 \cdot \vec{v}_1 - 2 \vec{S}_1 \times \vec{v}_1 \cdot \vec{a}_1 \vec{v}_1 \cdot \vec{v}_2 + 3 \vec{S}_1 \times \vec{v}_1 \cdot \vec{a}_1 \vec{v}_2 \cdot \vec{v}_2 + 6 \hat{n} \times \vec{S}_1 \cdot \vec{v}_1 \hat{n} \cdot \vec{a}_1 \vec{v}_2 \cdot \vec{v}_2 \Big) m_1 m_2 G^2 + \\
& \frac{1}{r^3} \left( -8 \hat{n} \times \vec{S}_1 \cdot \vec{v}_1 \vec{v}_1 \cdot \vec{v}_1 (\hat{n} \cdot \vec{v}_1)^2 - 6 \hat{n} \times \vec{S}_1 \cdot \vec{v}_1 \vec{v}_2 \cdot \vec{v}_2 (\hat{n} \cdot \vec{v}_1)^2 - 2 \vec{S}_1 \times \vec{v}_1 \cdot \vec{v}_2 \vec{v}_1 \cdot \vec{v}_1 \hat{n} \cdot \vec{v}_1 + \right. \\
& 8 \hat{n} \times \vec{S}_1 \cdot \vec{v}_1 \hat{n} \cdot \vec{v}_2 \vec{v}_1 \cdot \vec{v}_1 \hat{n} \cdot \vec{v}_1 - \frac{3}{2} \vec{S}_1 \times \vec{v}_1 \cdot \vec{v}_2 \vec{v}_2 \cdot \vec{v}_2 \hat{n} \cdot \vec{v}_1 + 6 \hat{n} \times \vec{S}_1 \cdot \vec{v}_1 \hat{n} \cdot \vec{v}_2 \vec{v}_2 \cdot \vec{v}_2 \hat{n} \cdot \vec{v}_1 + \\
& 2 \hat{n} \times \vec{S}_1 \cdot \vec{v}_1 (\vec{v}_1 \cdot \vec{v}_1)^2 - \frac{7}{16} \hat{n} \times \vec{S}_1 \cdot \vec{v}_1 (\vec{v}_2 \cdot \vec{v}_2)^2 - 2 \hat{n} \times \vec{S}_1 \cdot \vec{v}_1 \vec{v}_1 \cdot \vec{v}_1 \vec{v}_1 \cdot \vec{v}_2 + \\
& \left. \frac{3}{4} \hat{n} \times \vec{S}_1 \cdot \vec{v}_1 \vec{v}_1 \cdot \vec{v}_1 \vec{v}_2 \cdot \vec{v}_2 - \frac{3}{2} \hat{n} \times \vec{S}_1 \cdot \vec{v}_1 \vec{v}_1 \cdot \vec{v}_2 \vec{v}_2 \cdot \vec{v}_2 \right) m_1 m_2 G^2 \Big\}
\end{aligned}$$

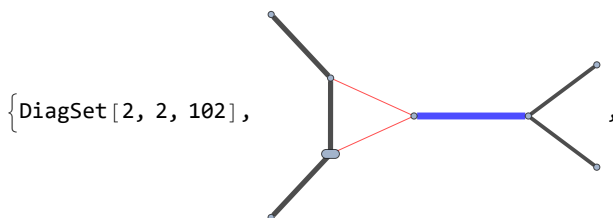

$$\begin{aligned}
& \frac{1}{r^2} G^2 m_1 m_2 \left( 2 (\hat{n} \cdot \vec{v}_2)^2 \vec{S}_1 \times \vec{v}_1 \cdot \vec{a}_1 + 2 \vec{v}_2 \cdot \vec{v}_2 \hat{n} \cdot \vec{v}_1 \hat{n} \times \vec{S}_1 \cdot \vec{a}_1 + 2 \vec{v}_2 \cdot \vec{v}_2 \hat{n} \cdot \vec{v}_1 \hat{n} \times \vec{S}_1 \cdot \vec{v}_1 \right) + \frac{1}{r^3} \\
& G^2 m_1 m_2 \left( -4 \vec{v}_2 \cdot \vec{v}_2 (\hat{n} \cdot \vec{v}_1)^2 \hat{n} \times \vec{S}_1 \cdot \vec{v}_1 - (\vec{v}_2 \cdot \vec{v}_2)^2 \hat{n} \times \vec{S}_1 \cdot \vec{v}_1 + 8 \vec{v}_1 \cdot \vec{v}_1 (\hat{n} \cdot \vec{v}_2)^2 \hat{n} \times \vec{S}_1 \cdot \vec{v}_1 - \right. \\
& \left. 4 \vec{v}_1 \cdot \vec{v}_1 \hat{n} \cdot \vec{v}_2 \vec{S}_1 \times \vec{v}_1 \cdot \vec{v}_2 + 2 \vec{v}_2 \cdot \vec{v}_2 (\hat{n} \cdot \vec{v}_2)^2 \hat{n} \times \vec{S}_1 \cdot \vec{v}_1 - \vec{v}_2 \cdot \vec{v}_2 \hat{n} \cdot \vec{v}_2 \vec{S}_1 \times \vec{v}_1 \cdot \vec{v}_2 - 2 \vec{v}_1 \cdot \vec{v}_1 \vec{v}_2 \cdot \vec{v}_2 \hat{n} \times \vec{S}_1 \cdot \vec{v}_1 \right) \Big\}
\end{aligned}$$

{DiagSet[2, 2, 103],

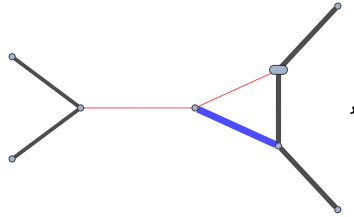

,

$$\frac{1}{r^2} G^2 m_1 m_2 \left( -8 (\hat{n} \cdot \vec{v}_1)^2 \vec{S}_1 \times \vec{v}_1 \cdot \vec{a}_1 - 8 \vec{v}_1 \cdot \vec{v}_1 \hat{n} \cdot \vec{v}_2 \hat{n} \times \vec{S}_1 \cdot \vec{a}_1 + \right. \\ \left. 4 \vec{v}_1 \cdot \vec{v}_1 \vec{S}_1 \times \vec{a}_1 \cdot \vec{v}_2 + 4 \vec{v}_1 \cdot \vec{v}_1 \vec{S}_1 \times \vec{v}_1 \cdot \vec{a}_1 - 8 \vec{v}_1 \cdot \vec{v}_1 \hat{n} \cdot \vec{v}_2 \hat{n} \times \vec{S}_1 \cdot \vec{v}_1 + 4 \vec{v}_1 \cdot \vec{v}_1 \vec{S}_1 \times \vec{v}_1 \cdot \vec{v}_2 \right) + \frac{1}{r^3} \\ G^2 m_1 m_2 \left( -24 \vec{v}_1 \cdot \vec{v}_1 (\hat{n} \cdot \vec{v}_1)^2 \hat{n} \times \vec{S}_1 \cdot \vec{v}_1 - 36 \vec{v}_2 \cdot \vec{v}_2 (\hat{n} \cdot \vec{v}_1)^2 \hat{n} \times \vec{S}_1 \cdot \vec{v}_1 - 6 \vec{v}_1 \cdot \vec{v}_1 \hat{n} \cdot \vec{v}_1 \vec{S}_1 \times \vec{v}_1 \cdot \vec{v}_2 + \right. \\ \left. 24 \vec{v}_1 \cdot \vec{v}_1 \hat{n} \cdot \vec{v}_2 \hat{n} \cdot \vec{v}_1 \hat{n} \times \vec{S}_1 \cdot \vec{v}_1 + 6 (\vec{v}_1 \cdot \vec{v}_1)^2 \hat{n} \times \vec{S}_1 \cdot \vec{v}_1 - 6 \vec{v}_1 \cdot \vec{v}_1 \vec{v}_1 \cdot \vec{v}_2 \hat{n} \times \vec{S}_1 \cdot \vec{v}_1 + 9 \vec{v}_1 \cdot \vec{v}_1 \vec{v}_2 \cdot \vec{v}_2 \hat{n} \times \vec{S}_1 \cdot \vec{v}_1 \right) \Big\}$$

{DiagSet[2, 2, 104],

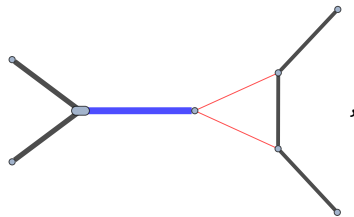

,

$$\frac{1}{r^2} G^2 m_2^2 \left( \frac{3}{8} (\hat{n} \cdot \vec{v}_1)^2 \vec{a}_1 \times \vec{S}_1 \cdot \vec{v}_1 - \frac{7}{8} \vec{a}_1 \cdot \vec{v}_1 \hat{n} \cdot \vec{v}_1 \hat{n} \times \vec{S}_1 \cdot \vec{v}_1 + \frac{5}{8} \vec{v}_1 \cdot \vec{v}_1 \hat{n} \cdot \vec{v}_1 \hat{n} \times \vec{a}_1 \cdot \vec{S}_1 + 3 \vec{v}_2 \cdot \vec{v}_2 \hat{n} \cdot \vec{v}_1 \hat{n} \times \vec{a}_1 \cdot \vec{S}_1 - \right. \\ \left. \frac{1}{2} (\hat{n} \cdot \vec{v}_2)^2 \vec{a}_1 \times \vec{S}_1 \cdot \vec{v}_1 - 12 \vec{a}_2 \cdot \vec{v}_2 \hat{n} \cdot \vec{v}_2 \hat{n} \times \vec{S}_1 \cdot \vec{v}_1 - \frac{1}{4} \vec{v}_1 \cdot \vec{v}_1 \hat{n} \cdot \vec{a}_1 \hat{n} \times \vec{S}_1 \cdot \vec{v}_1 - \frac{3}{2} \vec{v}_2 \cdot \vec{v}_2 \hat{n} \cdot \vec{a}_1 \hat{n} \times \vec{S}_1 \cdot \vec{v}_1 + 6 \vec{a}_2 \cdot \vec{v}_2 \right. \\ \left. \vec{S}_1 \times \vec{v}_1 \cdot \vec{v}_2 - \frac{3}{4} \vec{v}_1 \cdot \vec{v}_1 \vec{a}_1 \times \vec{S}_1 \cdot \vec{v}_1 - \vec{v}_2 \cdot \vec{v}_2 \vec{a}_1 \times \vec{S}_1 \cdot \vec{v}_1 - \frac{7}{16} \vec{v}_1 \cdot \vec{v}_1 \hat{n} \cdot \vec{v}_1 \hat{n} \times \vec{S}_1 \cdot \vec{v}_1 - \frac{9}{4} \vec{v}_2 \cdot \vec{v}_2 \hat{n} \cdot \vec{v}_1 \hat{n} \times \vec{S}_1 \cdot \vec{v}_1 \right) + \\ \frac{1}{r^3} G^2 m_2^2 \left( (\vec{v}_1 \cdot \vec{v}_1 (\hat{n} \cdot \vec{v}_1)^2 \hat{n} \times \vec{S}_1 \cdot \vec{v}_1 + 6 \vec{v}_2 \cdot \vec{v}_2 (\hat{n} \cdot \vec{v}_1)^2 \hat{n} \times \vec{S}_1 \cdot \vec{v}_1 - \frac{7}{16} (\vec{v}_1 \cdot \vec{v}_1)^2 \hat{n} \times \vec{S}_1 \cdot \vec{v}_1 + \right. \\ (\vec{v}_2 \cdot \vec{v}_2)^2 \hat{n} \times \vec{S}_1 \cdot \vec{v}_1 - \vec{v}_1 \cdot \vec{v}_1 (\hat{n} \cdot \vec{v}_2)^2 \hat{n} \times \vec{S}_1 \cdot \vec{v}_1 + \frac{1}{2} \vec{v}_1 \cdot \vec{v}_1 \hat{n} \cdot \vec{v}_2 \vec{S}_1 \times \vec{v}_1 \cdot \vec{v}_2 - \\ \left. 6 \vec{v}_2 \cdot \vec{v}_2 (\hat{n} \cdot \vec{v}_2)^2 \hat{n} \times \vec{S}_1 \cdot \vec{v}_1 + 3 \vec{v}_2 \cdot \vec{v}_2 \hat{n} \cdot \vec{v}_2 \vec{S}_1 \times \vec{v}_1 \cdot \vec{v}_2 - \frac{7}{4} \vec{v}_1 \cdot \vec{v}_1 \vec{v}_2 \cdot \vec{v}_2 \hat{n} \times \vec{S}_1 \cdot \vec{v}_1 \right) \Big\}$$

{DiagSet[2, 2, 105],

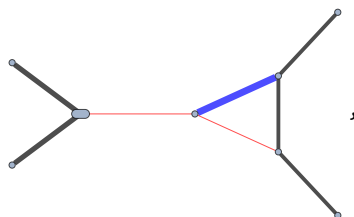

,

$$\frac{1}{r^2} G^2 m_2^2 \left( -8 (\hat{n} \cdot \vec{v}_2)^2 \vec{a}_1 \times \vec{S}_1 \cdot \vec{v}_1 + 8 \vec{v}_2 \cdot \vec{v}_2 \hat{n} \cdot \vec{v}_2 \hat{n} \times \vec{a}_1 \cdot \vec{S}_1 + 4 \vec{v}_2 \cdot \vec{v}_2 \vec{a}_1 \times \vec{S}_1 \cdot \vec{v}_1 - \right. \\ \left. 4 \vec{v}_2 \cdot \vec{v}_2 \vec{a}_1 \times \vec{S}_1 \cdot \vec{v}_2 - 8 \vec{v}_2 \cdot \vec{v}_2 \hat{n} \cdot \vec{v}_2 \hat{n} \times \vec{S}_1 \cdot \vec{v}_1 + 4 \vec{v}_2 \cdot \vec{v}_2 \vec{S}_1 \times \vec{v}_1 \cdot \vec{v}_2 \right) + \frac{1}{r^3} \\ G^2 m_2^2 \left( -16 \vec{v}_1 \cdot \vec{v}_1 (\hat{n} \cdot \vec{v}_2)^2 \hat{n} \times \vec{S}_1 \cdot \vec{v}_1 - 64 \vec{v}_2 \cdot \vec{v}_2 (\hat{n} \cdot \vec{v}_2)^2 \hat{n} \times \vec{S}_1 \cdot \vec{v}_1 + 8 \vec{v}_1 \cdot \vec{v}_1 \hat{n} \cdot \vec{v}_2 \vec{S}_1 \times \vec{v}_1 \cdot \vec{v}_2 + \right. \\ \left. 32 \vec{v}_2 \cdot \vec{v}_2 \hat{n} \cdot \vec{v}_2 \vec{S}_1 \times \vec{v}_1 \cdot \vec{v}_2 + 32 \vec{v}_2 \cdot \vec{v}_2 \hat{n} \cdot \vec{v}_1 \hat{n} \cdot \vec{v}_2 \hat{n} \times \vec{S}_1 \cdot \vec{v}_1 + 16 (\vec{v}_2 \cdot \vec{v}_2)^2 \hat{n} \times \vec{S}_1 \cdot \vec{v}_1 - \right. \\ \left. 8 \vec{v}_2 \cdot \vec{v}_2 \hat{n} \cdot \vec{v}_1 \vec{S}_1 \times \vec{v}_1 \cdot \vec{v}_2 + 4 \vec{v}_1 \cdot \vec{v}_1 \vec{v}_2 \cdot \vec{v}_2 \hat{n} \times \vec{S}_1 \cdot \vec{v}_1 - 8 \vec{v}_1 \cdot \vec{v}_2 \vec{v}_2 \cdot \vec{v}_2 \hat{n} \times \vec{S}_1 \cdot \vec{v}_1 \right) \Big\}$$

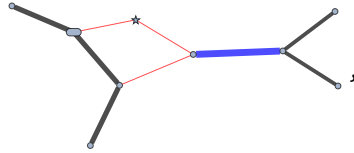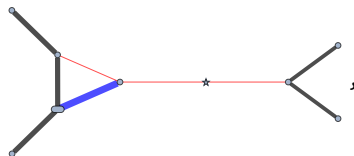

$$\left(\frac{7}{3}\vec{S_1}\times\vec{v_1}\cdot\vec{v_2}\left(\hat{n}\cdot\vec{v_1}\right)^2+3\vec{S_1}\times\vec{a_1}\cdot\vec{v_2}\left(\hat{n}\cdot\vec{v_1}\right)^2+\frac{1}{3}\vec{S_1}\times\vec{v_1}\cdot\vec{a_2}\left(\hat{n}\cdot\vec{v_1}\right)^2-\frac{4}{3}\hat{n}\times\vec{S_1}\cdot\vec{v_1}\hat{n}\cdot\vec{a_2}\left(\hat{n}\cdot\vec{v_1}\right)^2-\right.$$



$$\frac{1}{r^3} \left( -4 \hat{n} \times \vec{S}_1 \cdot \vec{v}_1 (\hat{n} \cdot \vec{v}_1)^4 - 4 \vec{S}_1 \times \vec{v}_1 \cdot \vec{v}_2 (\hat{n} \cdot \vec{v}_1)^3 + 24 \hat{n} \times \vec{S}_1 \cdot \vec{v}_1 \hat{n} \cdot \vec{v}_2 (\hat{n} \cdot \vec{v}_1)^3 + \right. \\ \left. 2 \hat{n} \times \vec{S}_1 \cdot \vec{v}_1 \vec{v}_1 \cdot \vec{v}_1 (\hat{n} \cdot \vec{v}_1)^2 - 12 \hat{n} \times \vec{S}_1 \cdot \vec{v}_1 \vec{v}_1 \cdot \vec{v}_2 (\hat{n} \cdot \vec{v}_1)^2 + 4 \vec{S}_1 \times \vec{v}_1 \cdot \vec{v}_2 \vec{v}_1 \cdot \vec{v}_1 \hat{n} \cdot \vec{v}_1 - \right. \\ \left. 16 \hat{n} \times \vec{S}_1 \cdot \vec{v}_1 \hat{n} \cdot \vec{v}_2 \vec{v}_1 \cdot \vec{v}_1 \hat{n} \cdot \vec{v}_1 + 4 \hat{n} \times \vec{S}_1 \cdot \vec{v}_1 \vec{v}_1 \cdot \vec{v}_1 \vec{v}_1 \cdot \vec{v}_2 \right) m_1 m_2 G^2 \}$$

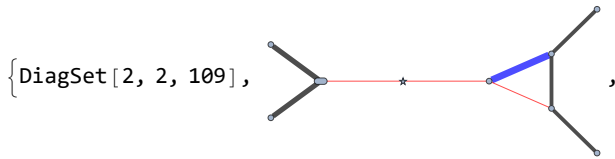

$$\frac{1}{r} G^2 \left( \frac{8}{3} \vec{S}_1 \times \vec{v}_1 \cdot \vec{v}_2 \hat{n} \cdot \vec{a}_2 - \frac{8}{3} \vec{a}_1 \times \vec{S}_1 \cdot \vec{v}_2 \hat{n} \cdot \vec{a}_2 - \frac{16}{3} \hat{n} \times \vec{S}_1 \cdot \vec{v}_1 \hat{n} \cdot \vec{v}_2 \hat{n} \cdot \vec{a}_2 + \frac{16}{3} \hat{n} \times \vec{a}_1 \cdot \vec{S}_1 \hat{n} \cdot \vec{v}_2 \hat{n} \cdot \vec{a}_2 + \right. \\ \left. \frac{8}{3} \vec{a}_1 \times \vec{a}_2 \cdot \vec{S}_1 \hat{n} \cdot \vec{v}_2 + \frac{8}{3} \vec{a}_2 \times \vec{S}_1 \cdot \vec{v}_1 \hat{n} \cdot \vec{v}_2 + \frac{8}{3} \hat{n} \times \vec{S}_1 \cdot \vec{v}_1 \vec{a}_2 \cdot \vec{v}_2 - \frac{8}{3} \hat{n} \times \vec{a}_1 \cdot \vec{S}_1 \vec{a}_2 \cdot \vec{v}_2 \right) m_2^2 + \frac{1}{r^2} \\ G^2 \left( -\frac{32}{3} \hat{n} \times \vec{S}_1 \cdot \vec{v}_1 (\hat{n} \cdot \vec{v}_2)^3 + \frac{32}{3} \hat{n} \times \vec{a}_1 \cdot \vec{S}_1 (\hat{n} \cdot \vec{v}_2)^3 + 8 \vec{S}_1 \times \vec{v}_1 \cdot \vec{v}_2 (\hat{n} \cdot \vec{v}_2)^2 - 8 \vec{a}_1 \times \vec{S}_1 \cdot \vec{v}_2 (\hat{n} \cdot \vec{v}_2)^2 - \right. \\ \left. \frac{16}{3} \vec{a}_2 \times \vec{S}_1 \cdot \vec{v}_1 \hat{n} \cdot \vec{v}_1 \hat{n} \cdot \vec{v}_2 + \frac{64}{3} \hat{n} \times \vec{S}_1 \cdot \vec{v}_1 \hat{n} \cdot \vec{a}_2 \hat{n} \cdot \vec{v}_1 \hat{n} \cdot \vec{v}_2 - \frac{16}{3} \hat{n} \times \vec{S}_1 \cdot \vec{v}_1 \vec{a}_2 \cdot \vec{v}_1 \hat{n} \cdot \vec{v}_2 + 8 \hat{n} \times \vec{S}_1 \cdot \vec{v}_1 \vec{v}_2 \cdot \vec{v}_2 \hat{n} \cdot \vec{v}_2 - \right. \\ \left. 8 \hat{n} \times \vec{a}_1 \cdot \vec{S}_1 \vec{v}_2 \cdot \vec{v}_2 \hat{n} \cdot \vec{v}_2 - \frac{16}{3} \vec{S}_1 \times \vec{v}_1 \cdot \vec{v}_2 \hat{n} \cdot \vec{a}_2 \hat{n} \cdot \vec{v}_1 + \frac{8}{3} \vec{S}_1 \times \vec{v}_1 \cdot \vec{v}_2 \vec{a}_2 \cdot \vec{v}_1 - \frac{16}{3} \hat{n} \times \vec{S}_1 \cdot \vec{v}_1 \hat{n} \cdot \vec{v}_1 \vec{a}_2 \cdot \vec{v}_2 + \right. \\ \left. \frac{8}{3} \vec{a}_2 \times \vec{S}_1 \cdot \vec{v}_1 \vec{v}_1 \cdot \vec{v}_2 - \frac{16}{3} \hat{n} \times \vec{S}_1 \cdot \vec{v}_1 \hat{n} \cdot \vec{a}_2 \vec{v}_1 \cdot \vec{v}_2 - 4 \vec{S}_1 \times \vec{v}_1 \cdot \vec{v}_2 \vec{v}_2 \cdot \vec{v}_2 + 4 \vec{a}_1 \times \vec{S}_1 \cdot \vec{v}_2 \vec{v}_2 \cdot \vec{v}_2 \right) m_2^2 + \frac{1}{r^3} \\ G^2 \left( 64 \hat{n} \times \vec{S}_1 \cdot \vec{v}_1 \hat{n} \cdot \vec{v}_1 (\hat{n} \cdot \vec{v}_2)^3 - 32 \vec{S}_1 \times \vec{v}_1 \cdot \vec{v}_2 \hat{n} \cdot \vec{v}_1 (\hat{n} \cdot \vec{v}_2)^2 - 32 \hat{n} \times \vec{S}_1 \cdot \vec{v}_1 \vec{v}_1 \cdot \vec{v}_2 (\hat{n} \cdot \vec{v}_2)^2 + 16 \vec{S}_1 \times \vec{v}_1 \cdot \vec{v}_2 \right. \\ \left. \vec{v}_1 \cdot \vec{v}_2 \hat{n} \cdot \vec{v}_2 - 32 \hat{n} \times \vec{S}_1 \cdot \vec{v}_1 \hat{n} \cdot \vec{v}_1 \vec{v}_2 \cdot \vec{v}_2 \hat{n} \cdot \vec{v}_2 + 8 \vec{S}_1 \times \vec{v}_1 \cdot \vec{v}_2 \hat{n} \cdot \vec{v}_1 \vec{v}_2 \cdot \vec{v}_2 + 8 \hat{n} \times \vec{S}_1 \cdot \vec{v}_1 \vec{v}_1 \cdot \vec{v}_2 \vec{v}_2 \cdot \vec{v}_2 \right) m_2^2 \}$$

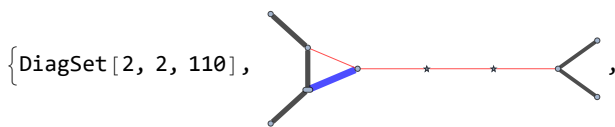

$$\frac{1}{r} \left( -\frac{1}{3} \hat{n} \times \vec{S}_1 \cdot \vec{a}_1 (\hat{n} \cdot \vec{v}_2)^2 - \frac{1}{6} \hat{n} \times \vec{S}_1 \cdot \vec{v}_1 (\hat{n} \cdot \vec{v}_2)^2 - \frac{1}{6} \hat{n} \times \vec{S}_1 \cdot \vec{a}_1 (\hat{n} \cdot \vec{v}_2)^2 + \frac{1}{3} \vec{S}_1 \times \vec{a}_1 \cdot \vec{v}_2 \hat{n} \cdot \vec{v}_2 + \frac{1}{6} \vec{S}_1 \times \vec{v}_1 \cdot \vec{v}_2 \hat{n} \cdot \vec{v}_2 + \right. \\ \left. \frac{1}{6} \vec{S}_1 \times \vec{a}_1 \cdot \vec{v}_2 \hat{n} \cdot \vec{v}_2 - \frac{1}{12} \vec{S}_1 \times \vec{v}_1 \cdot \vec{a}_2 \hat{n} \cdot \vec{a}_1 + \frac{1}{12} \vec{S}_1 \times \vec{v}_1 \cdot \vec{a}_1 \hat{n} \cdot \vec{a}_2 + \frac{1}{6} \hat{n} \times \vec{S}_1 \cdot \vec{v}_1 \hat{n} \cdot \vec{a}_1 \hat{n} \cdot \vec{a}_2 - \frac{1}{6} \vec{S}_1 \times \vec{v}_1 \cdot \vec{a}_2 \hat{n} \cdot \vec{v}_1 - \right. \\ \left. \frac{1}{6} \vec{S}_1 \times \vec{a}_1 \cdot \vec{a}_2 \hat{n} \cdot \vec{v}_1 + \frac{1}{3} \hat{n} \times \vec{S}_1 \cdot \vec{v}_1 \hat{n} \cdot \vec{a}_2 \hat{n} \cdot \vec{v}_1 + \frac{1}{3} \hat{n} \times \vec{S}_1 \cdot \vec{a}_1 \hat{n} \cdot \vec{a}_2 \hat{n} \cdot \vec{v}_1 - \frac{1}{12} \hat{n} \times \vec{S}_1 \cdot \vec{v}_1 \vec{a}_1 \cdot \vec{a}_2 - \right. \\ \left. \frac{1}{6} \hat{n} \times \vec{S}_1 \cdot \vec{v}_1 \vec{v}_1 \cdot \vec{a}_2 - \frac{1}{6} \hat{n} \times \vec{S}_1 \cdot \vec{a}_1 \vec{v}_1 \cdot \vec{a}_2 + \frac{1}{6} \hat{n} \times \vec{S}_1 \cdot \vec{a}_1 \vec{v}_2 \cdot \vec{v}_2 + \frac{1}{12} \hat{n} \times \vec{S}_1 \cdot \vec{v}_1 \vec{v}_2 \cdot \vec{v}_2 + \frac{1}{12} \hat{n} \times \vec{S}_1 \cdot \vec{a}_1 \vec{v}_2 \cdot \vec{v}_2 \right) \\ m_1 m_2 G^2 + \frac{1}{r^2} \left( \frac{1}{6} \vec{S}_1 \times \vec{v}_1 \cdot \vec{a}_2 (\hat{n} \cdot \vec{v}_1)^2 - \frac{2}{3} \hat{n} \times \vec{S}_1 \cdot \vec{v}_1 \hat{n} \cdot \vec{a}_2 (\hat{n} \cdot \vec{v}_1)^2 + \frac{4}{3} \hat{n} \times \vec{S}_1 \cdot \vec{v}_1 (\hat{n} \cdot \vec{v}_2)^2 \hat{n} \cdot \vec{v}_1 + \right. \\ \left. \frac{4}{3} \hat{n} \times \vec{S}_1 \cdot \vec{a}_1 (\hat{n} \cdot \vec{v}_2)^2 \hat{n} \cdot \vec{v}_1 - \frac{2}{3} \vec{S}_1 \times \vec{v}_1 \cdot \vec{v}_2 \hat{n} \cdot \vec{v}_2 \hat{n} \cdot \vec{v}_1 - \frac{2}{3} \vec{S}_1 \times \vec{a}_1 \cdot \vec{v}_2 \hat{n} \cdot \vec{v}_2 \hat{n} \cdot \vec{v}_1 + \frac{1}{3} \hat{n} \times \vec{S}_1 \cdot \vec{v}_1 \vec{v}_1 \cdot \vec{a}_2 \hat{n} \cdot \vec{v}_1 - \right. \\ \left. \frac{1}{3} \hat{n} \times \vec{S}_1 \cdot \vec{v}_1 \vec{v}_2 \cdot \vec{v}_2 \hat{n} \cdot \vec{v}_1 - \frac{1}{3} \hat{n} \times \vec{S}_1 \cdot \vec{a}_1 \vec{v}_2 \cdot \vec{v}_2 \hat{n} \cdot \vec{v}_1 + \frac{1}{6} \vec{S}_1 \times \vec{v}_1 \cdot \vec{a}_1 (\hat{n} \cdot \vec{v}_2)^2 + \frac{2}{3} \hat{n} \times \vec{S}_1 \cdot \vec{v}_1 \hat{n} \cdot \vec{a}_1 (\hat{n} \cdot \vec{v}_2)^2 - \right. \\ \left. \frac{1}{3} \vec{S}_1 \times \vec{v}_1 \cdot \vec{v}_2 \hat{n} \cdot \vec{a}_1 \hat{n} \cdot \vec{v}_2 + \frac{1}{6} \vec{S}_1 \times \vec{v}_1 \cdot \vec{v}_2 \vec{a}_1 \cdot \vec{v}_2 - \frac{1}{3} \hat{n} \times \vec{S}_1 \cdot \vec{v}_1 \hat{n} \cdot \vec{v}_2 \vec{a}_1 \cdot \vec{v}_2 - \frac{1}{12} \vec{S}_1 \times \vec{v}_1 \cdot \vec{a}_2 \vec{v}_1 \cdot \vec{v}_1 + \right. \\ \left. \frac{1}{6} \hat{n} \times \vec{S}_1 \cdot \vec{v}_1 \hat{n} \cdot \vec{a}_2 \vec{v}_1 \cdot \vec{v}_1 + \frac{1}{3} \vec{S}_1 \times \vec{v}_1 \cdot \vec{v}_2 \vec{v}_1 \cdot \vec{v}_2 + \frac{1}{3} \vec{S}_1 \times \vec{a}_1 \cdot \vec{v}_2 \vec{v}_1 \cdot \vec{v}_2 - \frac{2}{3} \hat{n} \times \vec{S}_1 \cdot \vec{v}_1 \hat{n} \cdot \vec{v}_2 \vec{v}_1 \cdot \vec{v}_2 - \right. \\ \left. \frac{2}{3} \hat{n} \times \vec{S}_1 \cdot \vec{a}_1 \hat{n} \cdot \vec{v}_2 \vec{v}_1 \cdot \vec{v}_2 - \frac{1}{12} \vec{S}_1 \times \vec{v}_1 \cdot \vec{a}_1 \vec{v}_2 \cdot \vec{v}_2 - \frac{1}{6} \hat{n} \times \vec{S}_1 \cdot \vec{v}_1 \hat{n} \cdot \vec{a}_1 \vec{v}_2 \cdot \vec{v}_2 \right) m_1 m_2 G^2 + \frac{1}{r^3} \\ \left( -4 \hat{n} \times \vec{S}_1 \cdot \vec{v}_1 (\hat{n} \cdot \vec{v}_2)^2 (\hat{n} \cdot \vec{v}_1)^2 + \frac{4}{3} \vec{S}_1 \times \vec{v}_1 \cdot \vec{v}_2 \hat{n} \cdot \vec{v}_2 (\hat{n} \cdot \vec{v}_1)^2 + \frac{2}{3} \hat{n} \times \vec{S}_1 \cdot \vec{v}_1 \vec{v}_2 \cdot \vec{v}_2 (\hat{n} \cdot \vec{v}_1)^2 - \right.$$

$$\begin{aligned} & \frac{2}{3} \vec{S}_1 \times \vec{v}_1 \cdot \vec{v}_2 \vec{v}_1 \cdot \vec{v}_2 \hat{n} \cdot \vec{v}_1 + \frac{8}{3} \hat{n} \times \vec{S}_1 \cdot \vec{v}_1 \hat{n} \cdot \vec{v}_2 \vec{v}_1 \cdot \vec{v}_2 \hat{n} \cdot \vec{v}_1 - \frac{1}{3} \hat{n} \times \vec{S}_1 \cdot \vec{v}_1 (\vec{v}_1 \cdot \vec{v}_2)^2 + \\ & \frac{2}{3} \hat{n} \times \vec{S}_1 \cdot \vec{v}_1 (\hat{n} \cdot \vec{v}_2)^2 \vec{v}_1 \cdot \vec{v}_1 - \frac{1}{3} \vec{S}_1 \times \vec{v}_1 \cdot \vec{v}_2 \hat{n} \cdot \vec{v}_2 \vec{v}_1 \cdot \vec{v}_1 - \frac{1}{6} \hat{n} \times \vec{S}_1 \cdot \vec{v}_1 \vec{v}_1 \cdot \vec{v}_1 \vec{v}_2 \cdot \vec{v}_2 \Big) m_1 m_2 G^2 + \\ & m_1 m_2 \left( -\frac{1}{6} \log\left(\frac{r}{R_\theta}\right) \frac{1}{\vec{S}_1 \times \vec{a}_1 \cdot \vec{a}_2} + \frac{1}{9} \frac{1}{\vec{S}_1 \times \vec{a}_1 \cdot \vec{a}_2} + \frac{1}{18} \frac{2}{\vec{S}_1 \times \vec{v}_1 \cdot \vec{a}_2} + \frac{1}{18} \frac{1}{\vec{S}_1 \times \vec{a}_1 \cdot \vec{a}_2} - \frac{1}{6} \hat{n} \times \vec{S}_1 \cdot \vec{a}_1 \hat{n} \cdot \vec{a}_2 - \right. \\ & \frac{1}{12} \hat{n} \times \vec{S}_1 \cdot \vec{v}_1 \hat{n} \cdot \vec{a}_2 - \frac{1}{12} \hat{n} \times \vec{S}_1 \cdot \vec{a}_1 \hat{n} \cdot \vec{a}_2 - \frac{1}{12} \frac{2}{\vec{S}_1 \times \vec{v}_1 \cdot \vec{a}_2} \log\left(\frac{r}{R_\theta}\right) - \\ & \left. \frac{1}{12} \frac{1}{\vec{S}_1 \times \vec{a}_1 \cdot \vec{a}_2} \log\left(\frac{r}{R_\theta}\right) + \frac{\frac{1}{12} \frac{1}{\vec{S}_1 \times \vec{a}_1 \cdot \vec{a}_2} + \frac{1}{24} \frac{2}{\vec{S}_1 \times \vec{v}_1 \cdot \vec{a}_2} + \frac{1}{24} \frac{1}{\vec{S}_1 \times \vec{a}_1 \cdot \vec{a}_2}}{\epsilon_d} \right) G^2 \Big\} \end{aligned}$$

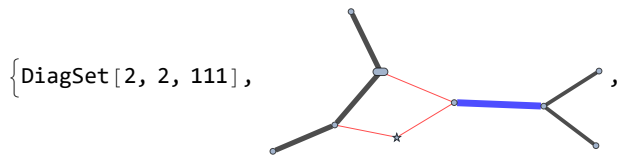

$$\begin{aligned} & \frac{1}{r^2} \left( \frac{1}{3} \vec{S}_1 \times \vec{v}_1 \cdot \vec{a}_1 (\hat{n} \cdot \vec{v}_2)^2 - \frac{2}{3} \hat{n} \times \vec{S}_1 \cdot \vec{v}_1 \hat{n} \cdot \vec{v}_1 (\hat{n} \cdot \vec{v}_2)^2 - \frac{2}{3} \hat{n} \times \vec{S}_1 \cdot \vec{a}_1 \hat{n} \cdot \vec{v}_1 (\hat{n} \cdot \vec{v}_2)^2 + \frac{1}{3} \frac{1}{\vec{S}_1 \times \vec{v}_1 \cdot \vec{v}_2} \hat{n} \cdot \vec{v}_1 \hat{n} \cdot \vec{v}_2 + \right. \\ & \frac{1}{3} \vec{S}_1 \times \vec{a}_1 \cdot \vec{v}_2 \hat{n} \cdot \vec{v}_1 \hat{n} \cdot \vec{v}_2 + \frac{1}{3} \vec{S}_1 \times \vec{v}_1 \cdot \vec{a}_2 \hat{n} \cdot \vec{v}_1 \hat{n} \cdot \vec{v}_2 - \frac{4}{3} \hat{n} \times \vec{S}_1 \cdot \vec{v}_1 \hat{n} \cdot \vec{a}_2 \hat{n} \cdot \vec{v}_1 \hat{n} \cdot \vec{v}_2 + \frac{7}{3} \hat{n} \times \vec{S}_1 \cdot \vec{v}_1 \vec{v}_1 \cdot \vec{a}_2 \hat{n} \cdot \vec{v}_2 + \\ & \frac{7}{3} \hat{n} \times \vec{S}_1 \cdot \vec{v}_1 \vec{v}_1 \cdot \vec{v}_2 \hat{n} \cdot \vec{v}_2 + \frac{7}{3} \hat{n} \times \vec{S}_1 \cdot \vec{a}_1 \vec{v}_1 \cdot \vec{v}_2 \hat{n} \cdot \vec{v}_2 + \frac{1}{3} \vec{S}_1 \times \vec{v}_1 \cdot \vec{v}_2 \hat{n} \cdot \vec{a}_2 \hat{n} \cdot \vec{v}_1 - \frac{2}{3} \vec{S}_1 \times \vec{v}_1 \cdot \vec{v}_2 \vec{v}_1 \cdot \vec{a}_2 - \\ & \frac{2}{3} \vec{S}_1 \times \vec{v}_1 \cdot \vec{v}_2 \vec{v}_1 \cdot \vec{v}_2 - \frac{2}{3} \vec{S}_1 \times \vec{a}_1 \cdot \vec{v}_2 \vec{v}_1 \cdot \vec{v}_2 - \frac{2}{3} \vec{S}_1 \times \vec{v}_1 \cdot \vec{a}_2 \vec{v}_1 \cdot \vec{v}_2 + \frac{7}{3} \hat{n} \times \vec{S}_1 \cdot \vec{v}_1 \hat{n} \cdot \vec{a}_2 \vec{v}_1 \cdot \vec{v}_2 - \\ & \left. \frac{2}{3} \hat{n} \times \vec{S}_1 \cdot \vec{v}_1 \hat{n} \cdot \vec{v}_1 \vec{v}_2 \cdot \vec{a}_2 - \frac{2}{3} \vec{S}_1 \times \vec{v}_1 \cdot \vec{a}_1 \vec{v}_2 \cdot \vec{v}_2 - \frac{1}{3} \hat{n} \times \vec{S}_1 \cdot \vec{v}_1 \hat{n} \cdot \vec{v}_1 \vec{v}_2 \cdot \vec{v}_2 - \frac{1}{3} \hat{n} \times \vec{S}_1 \cdot \vec{a}_1 \hat{n} \cdot \vec{v}_1 \vec{v}_2 \cdot \vec{v}_2 \right) m_1 m_2 G^2 + \\ & \frac{1}{r^3} \left( -4 \hat{n} \times \vec{S}_1 \cdot \vec{v}_1 \hat{n} \cdot \vec{v}_1 (\hat{n} \cdot \vec{v}_2)^3 + \frac{5}{2} \hat{n} \times \vec{S}_1 \cdot \vec{v}_1 (\hat{n} \cdot \vec{v}_1)^2 (\hat{n} \cdot \vec{v}_2)^2 + 2 \vec{S}_1 \times \vec{v}_1 \cdot \vec{v}_2 \hat{n} \cdot \vec{v}_1 (\hat{n} \cdot \vec{v}_2)^2 + \frac{5}{6} \hat{n} \times \vec{S}_1 \cdot \vec{v}_1 \right. \\ & \vec{v}_1 \cdot \vec{v}_1 (\hat{n} \cdot \vec{v}_2)^2 + 10 \hat{n} \times \vec{S}_1 \cdot \vec{v}_1 \vec{v}_1 \cdot \vec{v}_2 (\hat{n} \cdot \vec{v}_2)^2 - \frac{1}{3} \vec{S}_1 \times \vec{v}_1 \cdot \vec{v}_2 (\hat{n} \cdot \vec{v}_1)^2 \hat{n} \cdot \vec{v}_2 - \frac{2}{3} \vec{S}_1 \times \vec{v}_1 \cdot \vec{v}_2 \vec{v}_1 \cdot \vec{v}_1 \hat{n} \cdot \vec{v}_2 - \\ & 4 \vec{S}_1 \times \vec{v}_1 \cdot \vec{v}_2 \vec{v}_1 \cdot \vec{v}_2 \hat{n} \cdot \vec{v}_2 - \frac{26}{3} \hat{n} \times \vec{S}_1 \cdot \vec{v}_1 \hat{n} \cdot \vec{v}_1 \vec{v}_1 \cdot \vec{v}_2 \hat{n} \cdot \vec{v}_2 + \frac{4}{3} \hat{n} \times \vec{S}_1 \cdot \vec{v}_1 (\vec{v}_1 \cdot \vec{v}_2)^2 + \frac{5}{3} \vec{S}_1 \times \vec{v}_1 \cdot \vec{v}_2 \hat{n} \cdot \vec{v}_1 \vec{v}_1 \cdot \vec{v}_2 + \\ & \left. \frac{5}{6} \hat{n} \times \vec{S}_1 \cdot \vec{v}_1 (\hat{n} \cdot \vec{v}_1)^2 \vec{v}_2 \cdot \vec{v}_2 - \frac{5}{6} \hat{n} \times \vec{S}_1 \cdot \vec{v}_1 \vec{v}_1 \cdot \vec{v}_1 \vec{v}_2 \cdot \vec{v}_2 - 2 \hat{n} \times \vec{S}_1 \cdot \vec{v}_1 \vec{v}_1 \cdot \vec{v}_2 \vec{v}_2 \cdot \vec{v}_2 \right) m_1 m_2 G^2 \Big\} \end{aligned}$$

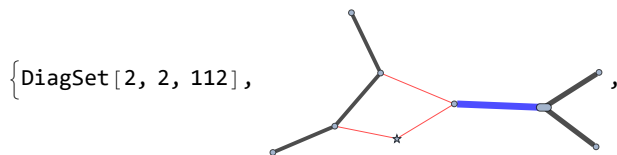

$$\begin{aligned} & \frac{1}{r} G^2 \left( -\frac{2}{3} \hat{n} \times \vec{S}_1 \cdot \vec{v}_1 (\hat{n} \cdot \vec{a}_2)^2 + \frac{1}{3} \frac{1}{\vec{S}_1 \times \vec{v}_1 \cdot \vec{v}_2} \hat{n} \cdot \vec{a}_2 - \frac{1}{3} \vec{a}_1 \times \vec{S}_1 \cdot \vec{v}_2 \hat{n} \cdot \vec{a}_2 + \frac{2}{3} \vec{a}_2 \times \vec{S}_1 \cdot \vec{v}_1 \hat{n} \cdot \vec{a}_2 - \frac{2}{3} \hat{n} \times \vec{S}_1 \cdot \vec{v}_1 \hat{n} \cdot \vec{v}_2 \hat{n} \cdot \vec{a}_2 + \right. \\ & \frac{2}{3} \hat{n} \times \vec{a}_1 \cdot \vec{S}_1 \hat{n} \cdot \vec{v}_2 \hat{n} \cdot \vec{a}_2 + \frac{1}{3} \vec{S}_1 \times \vec{v}_1 \cdot \vec{v}_2 \hat{n} \cdot \vec{a}_1 + \frac{5}{6} \frac{1}{\vec{S}_1 \times \vec{v}_1 \cdot \vec{v}_2} \hat{n} \cdot \vec{a}_1 - \vec{a}_1 \times \vec{S}_1 \cdot \vec{v}_2 \hat{n} \cdot \vec{a}_1 - \\ & \frac{2}{3} \frac{1}{\vec{a}_1 \times \vec{S}_1 \cdot \vec{v}_2} \hat{n} \cdot \vec{v}_1 + \frac{1}{2} \frac{2}{\vec{S}_1 \times \vec{v}_1 \cdot \vec{v}_2} \hat{n} \cdot \vec{v}_1 - \frac{7}{6} \frac{1}{\vec{a}_1 \times \vec{S}_1 \cdot \vec{v}_2} \hat{n} \cdot \vec{v}_1 + \frac{1}{6} \frac{1}{\vec{a}_1 \times \vec{S}_1 \cdot \vec{v}_1} \hat{n} \cdot \vec{v}_2 + \frac{1}{6} \frac{1}{\vec{a}_1 \times \vec{S}_1 \cdot \vec{v}_1} \hat{n} \cdot \vec{v}_2 + \\ & \frac{1}{3} \vec{a}_1 \times \vec{a}_2 \cdot \vec{S}_1 \hat{n} \cdot \vec{v}_2 + \frac{1}{3} \vec{a}_2 \times \vec{S}_1 \cdot \vec{v}_1 \hat{n} \cdot \vec{v}_2 - \frac{1}{6} \hat{n} \times \vec{S}_1 \cdot \vec{v}_1 \hat{n} \cdot \vec{a}_1 \hat{n} \cdot \vec{v}_2 - \frac{5}{12} \hat{n} \times \vec{S}_1 \cdot \vec{v}_1 \hat{n} \cdot \vec{a}_1 \hat{n} \cdot \vec{v}_2 + \\ & \left. \frac{1}{2} \hat{n} \times \vec{a}_1 \cdot \vec{S}_1 \hat{n} \cdot \vec{a}_1 \hat{n} \cdot \vec{v}_2 + \frac{1}{3} \hat{n} \times \vec{a}_1 \cdot \vec{S}_1 \hat{n} \cdot \vec{v}_1 \hat{n} \cdot \vec{v}_2 - \frac{1}{4} \hat{n} \times \vec{S}_1 \cdot \vec{v}_1 \hat{n} \cdot \vec{v}_1 \hat{n} \cdot \vec{v}_2 + \frac{7}{12} \hat{n} \times \vec{a}_1 \cdot \vec{S}_1 \hat{n} \cdot \vec{v}_1 \hat{n} \cdot \vec{v}_2 + \right. \end{aligned}$$

$$\begin{aligned} & \mathcal{G}^2 \left( -2 \hat{n} \times \vec{S}_1 \cdot \vec{v}_1 \left( \hat{n} \cdot \vec{v}_2 \right)^4 + \frac{4}{3} \vec{S}_1 \times \vec{v}_1 \cdot \vec{v}_2 \left( \hat{n} \cdot \vec{v}_2 \right)^3 + 4 \hat{n} \times \vec{S}_1 \cdot \vec{v}_1 \hat{n} \cdot \vec{v}_1 \left( \hat{n} \cdot \vec{v}_2 \right)^3 + 2 \hat{n} \times \vec{S}_1 \cdot \vec{v}_1 \left( \hat{n} \cdot \vec{v}_1 \right)^2 \left( \hat{n} \cdot \vec{v}_2 \right)^2 - \right. \\ & 2 \vec{S}_1 \times \vec{v}_1 \cdot \vec{v}_2 \hat{n} \cdot \vec{v}_1 \left( \hat{n} \cdot \vec{v}_2 \right)^2 + \frac{1}{6} \hat{n} \times \vec{S}_1 \cdot \vec{v}_1 \vec{v}_1 \cdot \vec{v}_1 \left( \hat{n} \cdot \vec{v}_2 \right)^2 - 2 \hat{n} \times \vec{S}_1 \cdot \vec{v}_1 \vec{v}_1 \cdot \vec{v}_2 \left( \hat{n} \cdot \vec{v}_2 \right)^2 + \\ & 7 \hat{n} \times \vec{S}_1 \cdot \vec{v}_1 \vec{v}_2 \cdot \vec{v}_2 \left( \hat{n} \cdot \vec{v}_2 \right)^2 - 4 \hat{n} \times \vec{S}_1 \cdot \vec{v}_1 \left( \hat{n} \cdot \vec{v}_1 \right)^3 \hat{n} \cdot \vec{v}_2 - \frac{5}{3} \vec{S}_1 \times \vec{v}_1 \cdot \vec{v}_2 \left( \hat{n} \cdot \vec{v}_1 \right)^2 \hat{n} \cdot \vec{v}_2 + \\ & \frac{1}{6} \vec{S}_1 \times \vec{v}_1 \cdot \vec{v}_2 \vec{v}_1 \cdot \vec{v}_1 \hat{n} \cdot \vec{v}_2 + \hat{n} \times \vec{S}_1 \cdot \vec{v}_1 \hat{n} \cdot \vec{v}_1 \vec{v}_1 \cdot \vec{v}_1 \hat{n} \cdot \vec{v}_2 + \vec{S}_1 \times \vec{v}_1 \cdot \vec{v}_2 \vec{v}_1 \cdot \vec{v}_2 \hat{n} \cdot \vec{v}_2 - \\ & \frac{13}{3} \hat{n} \times \vec{S}_1 \cdot \vec{v}_1 \hat{n} \cdot \vec{v}_1 \vec{v}_1 \cdot \vec{v}_2 \hat{n} \cdot \vec{v}_2 - 5 \vec{S}_1 \times \vec{v}_1 \cdot \vec{v}_2 \vec{v}_2 \cdot \vec{v}_2 \hat{n} \cdot \vec{v}_2 - 10 \hat{n} \times \vec{S}_1 \cdot \vec{v}_1 \hat{n} \cdot \vec{v}_1 \vec{v}_2 \cdot \vec{v}_2 \hat{n} \cdot \vec{v}_2 - \\ & 6 \hat{n} \times \vec{S}_1 \cdot \vec{v}_2 \hat{n} \cdot \vec{v}_1 \vec{v}_2 \cdot \vec{v}_2 \hat{n} \cdot \vec{v}_2 + \frac{5}{3} \vec{S}_1 \times \vec{v}_1 \cdot \vec{v}_2 \left( \hat{n} \cdot \vec{v}_1 \right)^3 + \frac{2}{3} \hat{n} \times \vec{S}_1 \cdot \vec{v}_1 \left( \vec{v}_1 \cdot \vec{v}_2 \right)^2 - \frac{3}{2} \hat{n} \times \vec{S}_1 \cdot \vec{v}_1 \left( \vec{v}_2 \cdot \vec{v}_2 \right)^2 - \\ & \vec{S}_1 \times \vec{v}_1 \cdot \vec{v}_2 \hat{n} \cdot \vec{v}_1 \vec{v}_1 \cdot \vec{v}_1 + 5 \hat{n} \times \vec{S}_1 \cdot \vec{v}_1 \left( \hat{n} \cdot \vec{v}_1 \right)^2 \vec{v}_1 \cdot \vec{v}_2 + \frac{4}{3} \vec{S}_1 \times \vec{v}_1 \cdot \vec{v}_2 \hat{n} \cdot \vec{v}_1 \vec{v}_1 \cdot \vec{v}_2 - \hat{n} \times \vec{S}_1 \cdot \vec{v}_1 \vec{v}_1 \cdot \vec{v}_1 \vec{v}_1 \cdot \vec{v}_2 + \\ & \frac{2}{3} \hat{n} \times \vec{S}_1 \cdot \vec{v}_1 \left( \hat{n} \cdot \vec{v}_1 \right)^2 \vec{v}_2 \cdot \vec{v}_2 + 6 \hat{n} \times \vec{S}_1 \cdot \vec{v}_2 \left( \hat{n} \cdot \vec{v}_1 \right)^2 \vec{v}_2 \cdot \vec{v}_2 + \frac{11}{2} \vec{S}_1 \times \vec{v}_1 \cdot \vec{v}_2 \hat{n} \cdot \vec{v}_1 \vec{v}_2 \cdot \vec{v}_2 - \\ & \left. \frac{5}{12} \hat{n} \times \vec{S}_1 \cdot \vec{v}_1 \vec{v}_1 \cdot \vec{v}_1 \vec{v}_2 \cdot \vec{v}_2 - \frac{3}{2} \hat{n} \times \vec{S}_1 \cdot \vec{v}_2 \vec{v}_1 \cdot \vec{v}_1 \vec{v}_2 \cdot \vec{v}_2 + \frac{5}{2} \hat{n} \times \vec{S}_1 \cdot \vec{v}_1 \vec{v}_1 \cdot \vec{v}_2 \vec{v}_2 \cdot \vec{v}_2 \right) m_2^2 \} \end{aligned}$$



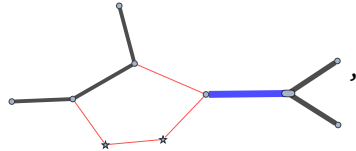

[illegible]

$$\begin{aligned}
& \frac{3}{4} \hat{n} \times \vec{S}_1 \cdot \vec{v}_2 \hat{n} \cdot \vec{v}_2 \vec{a}_2 \cdot \vec{v}_1 - \frac{1}{4} \vec{S}_1 \times \vec{v}_1 \cdot \vec{v}_2 \vec{a}_2 \cdot \vec{v}_2 + \frac{1}{2} \hat{n} \times \vec{S}_1 \cdot \vec{v}_1 \hat{n} \cdot \vec{v}_2 \vec{a}_2 \cdot \vec{v}_2 - \frac{5}{12} \vec{a}_2 \times \vec{S}_1 \cdot \vec{v}_1 \vec{v}_1 \cdot \vec{v}_1 + \\
& \frac{1}{3} \vec{a}_2 \times \vec{S}_1 \cdot \vec{v}_2 \vec{v}_1 \cdot \vec{v}_1 - \frac{1}{6} \hat{n} \times \vec{S}_1 \cdot \vec{v}_1 \hat{n} \cdot \vec{a}_2 \vec{v}_1 \cdot \vec{v}_1 + \frac{1}{12} \hat{n} \times \vec{S}_1 \cdot \vec{v}_2 \hat{n} \cdot \vec{a}_2 \vec{v}_1 \cdot \vec{v}_1 - \frac{1}{6} \hat{n} \times \vec{S}_1 \cdot \vec{v}_2 \hat{n} \cdot \vec{v}_2 \vec{v}_1 \cdot \vec{v}_1 - \\
& \frac{3}{4} \hat{n} \times \vec{a}_2 \cdot \vec{S}_1 \hat{n} \cdot \vec{v}_2 \vec{v}_1 \cdot \vec{v}_1 + \frac{1}{2} \vec{S}_1 \times \vec{v}_1 \cdot \vec{v}_2 \vec{v}_1 \cdot \vec{v}_2 - \frac{1}{6} \vec{a}_1 \times \vec{S}_1 \cdot \vec{v}_2 \vec{v}_1 \cdot \vec{v}_2 + \frac{1}{4} \vec{a}_2 \times \vec{S}_1 \cdot \vec{v}_1 \vec{v}_1 \cdot \vec{v}_2 + \frac{1}{3} \vec{a}_2 \times \vec{S}_1 \cdot \vec{v}_2 \vec{v}_1 \cdot \vec{v}_2 + \\
& \frac{1}{2} \hat{n} \times \vec{S}_1 \cdot \vec{v}_2 \hat{n} \cdot \vec{a}_1 \vec{v}_1 \cdot \vec{v}_2 + \frac{1}{4} \hat{n} \times \vec{S}_1 \cdot \vec{v}_1 \hat{n} \cdot \vec{a}_2 \vec{v}_1 \cdot \vec{v}_2 - \frac{3}{4} \hat{n} \times \vec{S}_1 \cdot \vec{v}_2 \hat{n} \cdot \vec{a}_2 \vec{v}_1 \cdot \vec{v}_2 + \frac{1}{6} \hat{n} \times \vec{S}_1 \cdot \vec{v}_1 \hat{n} \cdot \vec{v}_2 \vec{v}_1 \cdot \vec{v}_2 - \\
& \frac{5}{12} \hat{n} \times \vec{S}_1 \cdot \vec{v}_2 \hat{n} \cdot \vec{v}_2 \vec{v}_1 \cdot \vec{v}_2 - \frac{1}{6} \hat{n} \times \vec{a}_1 \cdot \vec{S}_1 \hat{n} \cdot \vec{v}_2 \vec{v}_1 \cdot \vec{v}_2 + \frac{1}{12} \hat{n} \times \vec{a}_2 \cdot \vec{S}_1 \hat{n} \cdot \vec{v}_2 \vec{v}_1 \cdot \vec{v}_2 - \frac{1}{24} \vec{S}_1 \times \vec{v}_1 \cdot \vec{v}_2 \vec{v}_2 \cdot \vec{v}_2 + \\
& \frac{5}{24} \vec{a}_1 \times \vec{S}_1 \cdot \vec{v}_1 \vec{v}_2 \cdot \vec{v}_2 + \frac{1}{24} \vec{a}_1 \times \vec{S}_1 \cdot \vec{v}_2 \vec{v}_2 \cdot \vec{v}_2 + \frac{1}{24} \vec{a}_2 \times \vec{S}_1 \cdot \vec{v}_1 \vec{v}_2 \cdot \vec{v}_2 + \frac{5}{12} \hat{n} \times \vec{S}_1 \cdot \vec{v}_1 \hat{n} \cdot \vec{a}_1 \vec{v}_2 \cdot \vec{v}_2 - \\
& \frac{7}{12} \hat{n} \times \vec{S}_1 \cdot \vec{v}_2 \hat{n} \cdot \vec{a}_1 \vec{v}_2 \cdot \vec{v}_2 - \frac{1}{2} \hat{n} \times \vec{S}_1 \cdot \vec{v}_1 \hat{n} \cdot \vec{a}_2 \vec{v}_2 \cdot \vec{v}_2 - \frac{1}{2} \hat{n} \times \vec{S}_1 \cdot \vec{v}_1 \hat{n} \cdot \vec{v}_2 \vec{v}_2 \cdot \vec{v}_2 + \frac{1}{2} \hat{n} \times \vec{a}_1 \cdot \vec{S}_1 \hat{n} \cdot \vec{v}_2 \vec{v}_2 \cdot \vec{v}_2 \Big) m_2^2 + \\
& \frac{1}{r^3} G^2 \left( \frac{5}{16} \hat{n} \times \vec{S}_1 \cdot \vec{v}_1 (\hat{n} \cdot \vec{v}_2)^4 - \frac{1}{2} \vec{S}_1 \times \vec{v}_1 \cdot \vec{v}_2 (\hat{n} \cdot \vec{v}_2)^3 - \hat{n} \times \vec{S}_1 \cdot \vec{v}_1 \hat{n} \cdot \vec{v}_1 (\hat{n} \cdot \vec{v}_2)^3 - \frac{7}{4} \hat{n} \times \vec{S}_1 \cdot \vec{v}_2 \hat{n} \cdot \vec{v}_1 (\hat{n} \cdot \vec{v}_2)^3 + \right. \\
& \hat{n} \times \vec{S}_1 \cdot \vec{v}_1 (\hat{n} \cdot \vec{v}_1)^2 (\hat{n} \cdot \vec{v}_2)^2 + 4 \hat{n} \times \vec{S}_1 \cdot \vec{v}_2 (\hat{n} \cdot \vec{v}_1)^2 (\hat{n} \cdot \vec{v}_2)^2 + \frac{11}{6} \vec{S}_1 \times \vec{v}_1 \cdot \vec{v}_2 \hat{n} \cdot \vec{v}_1 (\hat{n} \cdot \vec{v}_2)^2 - \\
& \frac{1}{6} \hat{n} \times \vec{S}_1 \cdot \vec{v}_1 \vec{v}_1 \cdot \vec{v}_1 (\hat{n} \cdot \vec{v}_2)^2 - \frac{2}{3} \hat{n} \times \vec{S}_1 \cdot \vec{v}_2 \vec{v}_1 \cdot \vec{v}_1 (\hat{n} \cdot \vec{v}_2)^2 + \frac{1}{2} \hat{n} \times \vec{S}_1 \cdot \vec{v}_1 \vec{v}_1 \cdot \vec{v}_2 (\hat{n} \cdot \vec{v}_2)^2 - \\
& \frac{1}{4} \hat{n} \times \vec{S}_1 \cdot \vec{v}_2 \vec{v}_1 \cdot \vec{v}_2 (\hat{n} \cdot \vec{v}_2)^2 - \frac{7}{8} \hat{n} \times \vec{S}_1 \cdot \vec{v}_1 \vec{v}_2 \cdot \vec{v}_2 (\hat{n} \cdot \vec{v}_2)^2 - 2 \hat{n} \times \vec{S}_1 \cdot \vec{v}_2 (\hat{n} \cdot \vec{v}_1)^3 \hat{n} \cdot \vec{v}_2 - \\
& \frac{4}{3} \vec{S}_1 \times \vec{v}_1 \cdot \vec{v}_2 (\hat{n} \cdot \vec{v}_1)^2 \hat{n} \cdot \vec{v}_2 + \frac{1}{3} \vec{S}_1 \times \vec{v}_1 \cdot \vec{v}_2 \vec{v}_1 \cdot \vec{v}_1 \hat{n} \cdot \vec{v}_2 + \hat{n} \times \vec{S}_1 \cdot \vec{v}_2 \hat{n} \cdot \vec{v}_1 \vec{v}_1 \cdot \vec{v}_1 \hat{n} \cdot \vec{v}_2 - \\
& \frac{1}{6} \vec{S}_1 \times \vec{v}_1 \cdot \vec{v}_2 \vec{v}_1 \cdot \vec{v}_2 \hat{n} \cdot \vec{v}_2 - \frac{2}{3} \hat{n} \times \vec{S}_1 \cdot \vec{v}_1 \hat{n} \cdot \vec{v}_1 \vec{v}_1 \cdot \vec{v}_2 \hat{n} \cdot \vec{v}_2 + \frac{1}{3} \hat{n} \times \vec{S}_1 \cdot \vec{v}_2 \hat{n} \cdot \vec{v}_1 \vec{v}_1 \cdot \vec{v}_2 \hat{n} \cdot \vec{v}_2 + \\
& 2 \hat{n} \times \vec{S}_1 \cdot \vec{v}_1 \hat{n} \cdot \vec{v}_1 \vec{v}_2 \cdot \vec{v}_2 \hat{n} \cdot \vec{v}_2 - \frac{7}{4} \hat{n} \times \vec{S}_1 \cdot \vec{v}_2 \hat{n} \cdot \vec{v}_1 \vec{v}_2 \cdot \vec{v}_2 \hat{n} \cdot \vec{v}_2 + \frac{1}{12} \hat{n} \times \vec{S}_1 \cdot \vec{v}_1 (\vec{v}_1 \cdot \vec{v}_2)^2 - \\
& \frac{5}{12} \hat{n} \times \vec{S}_1 \cdot \vec{v}_2 (\vec{v}_1 \cdot \vec{v}_2)^2 + \frac{1}{16} \hat{n} \times \vec{S}_1 \cdot \vec{v}_1 (\vec{v}_2 \cdot \vec{v}_2)^2 - 2 \hat{n} \times \vec{S}_1 \cdot \vec{v}_2 (\hat{n} \cdot \vec{v}_1)^2 \vec{v}_1 \cdot \vec{v}_2 - \\
& \frac{5}{6} \vec{S}_1 \times \vec{v}_1 \cdot \vec{v}_2 \hat{n} \cdot \vec{v}_1 \vec{v}_1 \cdot \vec{v}_2 + \frac{1}{2} \hat{n} \times \vec{S}_1 \cdot \vec{v}_2 \vec{v}_1 \cdot \vec{v}_1 \vec{v}_1 \cdot \vec{v}_2 - \frac{5}{3} \hat{n} \times \vec{S}_1 \cdot \vec{v}_1 (\hat{n} \cdot \vec{v}_1)^2 \vec{v}_2 \cdot \vec{v}_2 + \\
& \frac{7}{3} \hat{n} \times \vec{S}_1 \cdot \vec{v}_2 (\hat{n} \cdot \vec{v}_1)^2 \vec{v}_2 \cdot \vec{v}_2 + \frac{2}{3} \vec{S}_1 \times \vec{v}_1 \cdot \vec{v}_2 \hat{n} \cdot \vec{v}_1 \vec{v}_2 \cdot \vec{v}_2 + \frac{5}{12} \hat{n} \times \vec{S}_1 \cdot \vec{v}_1 \vec{v}_1 \cdot \vec{v}_1 \vec{v}_2 \cdot \vec{v}_2 - \\
& \left. \frac{7}{12} \hat{n} \times \vec{S}_1 \cdot \vec{v}_2 \vec{v}_1 \cdot \vec{v}_1 \vec{v}_2 \cdot \vec{v}_2 - \frac{1}{2} \hat{n} \times \vec{S}_1 \cdot \vec{v}_1 \vec{v}_1 \cdot \vec{v}_2 \vec{v}_2 \cdot \vec{v}_2 + \frac{1}{4} \hat{n} \times \vec{S}_1 \cdot \vec{v}_2 \vec{v}_1 \cdot \vec{v}_2 \vec{v}_2 \cdot \vec{v}_2 \right) m_2^2 + \\
& G^2 \left( -\frac{1}{12} \log\left(\frac{r}{R_\theta}\right) \frac{1}{\vec{a}_1 \times \vec{a}_2 \cdot \vec{S}_1} + \frac{17}{144} \frac{1}{\vec{a}_1 \times \vec{a}_2 \cdot \vec{S}_1} + \frac{17}{72} \frac{1}{\vec{a}_1 \times \vec{a}_2 \cdot \vec{S}_1} + \frac{17}{144} \frac{2}{\vec{a}_2 \times \vec{S}_1 \cdot \vec{v}_1} - \frac{1}{6} \hat{n} \times \vec{a}_2 \cdot \vec{S}_1 \hat{n} \cdot \vec{a}_1 - \right. \\
& \frac{1}{3} \hat{n} \times \vec{a}_2 \cdot \vec{S}_1 \hat{n} \cdot \vec{a}_1 - \frac{1}{12} \hat{n} \times \vec{a}_1 \cdot \vec{S}_1 \hat{n} \cdot \vec{a}_2 + \frac{1}{12} \hat{n} \times \vec{S}_1 \cdot \vec{v}_1 \hat{n} \cdot \vec{a}_2 - \frac{1}{6} \hat{n} \times \vec{a}_1 \cdot \vec{S}_1 \hat{n} \cdot \vec{a}_2 - \frac{1}{6} \hat{n} \times \vec{a}_2 \cdot \vec{S}_1 \hat{n} \cdot \vec{v}_1 - \\
& \left. \frac{1}{6} \vec{a}_1 \times \vec{a}_2 \cdot \vec{S}_1 \log\left(\frac{r}{R_\theta}\right) - \frac{1}{12} \vec{a}_2 \times \vec{S}_1 \cdot \vec{v}_1 \log\left(\frac{r}{R_\theta}\right) + \frac{\frac{1}{24} \frac{1}{\vec{a}_1 \times \vec{a}_2 \cdot \vec{S}_1} + \frac{1}{12} \frac{1}{\vec{a}_1 \times \vec{a}_2 \cdot \vec{S}_1} + \frac{1}{24} \frac{2}{\vec{a}_2 \times \vec{S}_1 \cdot \vec{v}_1}}{\epsilon_d} \right) m_2^2 \Big\}
\end{aligned}$$

{DiagSet[2, 2, 114],

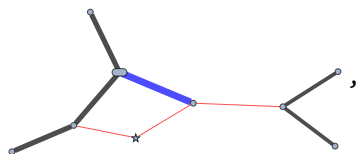

$$\frac{1}{r} \left( -\frac{7}{3} \hat{n} \times \vec{S}_1 \cdot \vec{a}_1 (\hat{n} \cdot \vec{v}_1)^2 - \hat{n} \times \vec{S}_1 \cdot \vec{v}_1 (\hat{n} \cdot \vec{v}_1)^2 - \frac{4}{3} \hat{n} \times \vec{S}_1 \cdot \vec{a}_1 (\hat{n} \cdot \vec{v}_1)^2 - \frac{13}{4} \frac{1}{\vec{S}_1 \times \vec{v}_1 \cdot \vec{a}_1} \hat{n} \cdot \vec{v}_1 - \right.$$

$$\begin{aligned}
& 2 \vec{S}_1 \times \vec{v}_1 \cdot \frac{1}{\vec{a}_1} \hat{n} \cdot \vec{v}_1 - \frac{2}{3} \hat{n} \times \vec{S}_1 \cdot \vec{v}_1 \hat{n} \cdot \frac{1}{\vec{a}_1} \hat{n} \cdot \vec{v}_1 - \frac{5}{3} \hat{n} \times \vec{S}_1 \cdot \vec{v}_1 \hat{n} \cdot \vec{a}_1 \hat{n} \cdot \vec{v}_1 - 2 \hat{n} \times \vec{S}_1 \cdot \vec{a}_1 \hat{n} \cdot \vec{a}_1 \hat{n} \cdot \vec{v}_1 - \\
& \frac{1}{3} \vec{S}_1 \times \vec{v}_1 \cdot \vec{v}_2 \hat{n} \cdot \vec{a}_1 - \frac{1}{3} \vec{S}_1 \times \vec{a}_1 \cdot \vec{v}_2 \hat{n} \cdot \vec{a}_1 - \frac{5}{2} \vec{S}_1 \times \vec{v}_1 \cdot \vec{a}_1 \hat{n} \cdot \vec{a}_1 - \frac{1}{3} \vec{S}_1 \times \vec{v}_1 \cdot \vec{a}_2 \hat{n} \cdot \vec{a}_1 + \frac{2}{3} \vec{S}_1 \times \vec{v}_1 \cdot \vec{a}_1 \hat{n} \cdot \vec{a}_2 + \\
& \frac{2}{3} \hat{n} \times \vec{S}_1 \cdot \vec{v}_1 \hat{n} \cdot \vec{a}_1 \hat{n} \cdot \vec{a}_2 + \frac{2}{3} \vec{S}_1 \times \vec{v}_1 \cdot \vec{a}_1 \hat{n} \cdot \vec{v}_2 + \frac{2}{3} \hat{n} \times \vec{S}_1 \cdot \vec{v}_1 \hat{n} \cdot \vec{a}_1 \hat{n} \cdot \vec{v}_2 + \frac{2}{3} \hat{n} \times \vec{S}_1 \cdot \vec{a}_1 \hat{n} \cdot \vec{a}_1 \hat{n} \cdot \vec{v}_2 - \\
& \frac{1}{3} \hat{n} \times \vec{S}_1 \cdot \vec{v}_1 \vec{a}_1 \cdot \vec{a}_2 - \frac{1}{3} \hat{n} \times \vec{S}_1 \cdot \vec{v}_1 \vec{a}_1 \cdot \vec{v}_2 - \frac{1}{3} \hat{n} \times \vec{S}_1 \cdot \vec{a}_1 \vec{a}_1 \cdot \vec{v}_2 + \frac{5}{6} \hat{n} \times \vec{S}_1 \cdot \vec{v}_1 \vec{v}_1 \cdot \frac{1}{\vec{a}_1} + \frac{43}{12} \hat{n} \times \vec{S}_1 \cdot \vec{v}_1 \vec{v}_1 \cdot \vec{a}_1 + \\
& 4 \hat{n} \times \vec{S}_1 \cdot \vec{a}_1 \vec{v}_1 \cdot \vec{a}_1 + \frac{35}{12} \hat{n} \times \vec{S}_1 \cdot \vec{a}_1 \vec{v}_1 \cdot \vec{v}_1 + \frac{5}{4} \hat{n} \times \vec{S}_1 \cdot \vec{v}_1 \vec{v}_1 \cdot \vec{v}_1 + \frac{5}{3} \hat{n} \times \vec{S}_1 \cdot \frac{1}{\vec{a}_1} \vec{v}_1 \cdot \vec{v}_1 \Big) m_1 m_2 G^2 + \\
& \frac{1}{r^2} \Big( \frac{5}{3} \hat{n} \times \vec{S}_1 \cdot \vec{v}_1 (\hat{n} \cdot \vec{v}_1)^3 + 2 \hat{n} \times \vec{S}_1 \cdot \vec{a}_1 (\hat{n} \cdot \vec{v}_1)^3 + \frac{7}{6} \vec{S}_1 \times \vec{v}_1 \cdot \vec{v}_2 (\hat{n} \cdot \vec{v}_1)^2 + \frac{3}{2} \vec{S}_1 \times \vec{a}_1 \cdot \vec{v}_2 (\hat{n} \cdot \vec{v}_1)^2 + \\
& \frac{17}{8} \vec{S}_1 \times \vec{v}_1 \cdot \vec{a}_1 (\hat{n} \cdot \vec{v}_1)^2 + \frac{1}{6} \vec{S}_1 \times \vec{v}_1 \cdot \vec{a}_2 (\hat{n} \cdot \vec{v}_1)^2 + 2 \hat{n} \times \vec{S}_1 \cdot \vec{v}_1 \hat{n} \cdot \vec{a}_1 (\hat{n} \cdot \vec{v}_1)^2 - \frac{2}{3} \hat{n} \times \vec{S}_1 \cdot \vec{v}_1 \hat{n} \cdot \vec{a}_2 (\hat{n} \cdot \vec{v}_1)^2 - \\
& \frac{14}{3} \hat{n} \times \vec{S}_1 \cdot \vec{v}_1 \hat{n} \cdot \vec{v}_2 (\hat{n} \cdot \vec{v}_1)^2 - 6 \hat{n} \times \vec{S}_1 \cdot \vec{a}_1 \hat{n} \cdot \vec{v}_2 (\hat{n} \cdot \vec{v}_1)^2 + \frac{7}{6} \vec{S}_1 \times \vec{v}_1 \cdot \vec{v}_2 \hat{n} \cdot \vec{a}_1 \hat{n} \cdot \vec{v}_1 - \frac{13}{3} \vec{S}_1 \times \vec{v}_1 \cdot \vec{a}_1 \hat{n} \cdot \vec{v}_2 \hat{n} \cdot \vec{v}_1 - \\
& \frac{14}{3} \hat{n} \times \vec{S}_1 \cdot \vec{v}_1 \hat{n} \cdot \vec{a}_1 \hat{n} \cdot \vec{v}_2 \hat{n} \cdot \vec{v}_1 + \frac{7}{6} \hat{n} \times \vec{S}_1 \cdot \vec{v}_1 \vec{a}_1 \cdot \vec{v}_2 \hat{n} \cdot \vec{v}_1 - \frac{5}{8} \hat{n} \times \vec{S}_1 \cdot \vec{v}_1 \vec{v}_1 \cdot \vec{a}_1 \hat{n} \cdot \vec{v}_1 + \\
& \frac{1}{3} \hat{n} \times \vec{S}_1 \cdot \vec{v}_1 \vec{v}_1 \cdot \vec{a}_2 \hat{n} \cdot \vec{v}_1 - \frac{17}{4} \hat{n} \times \vec{S}_1 \cdot \vec{v}_1 \vec{v}_1 \cdot \vec{v}_1 \hat{n} \cdot \vec{v}_1 - \frac{21}{8} \hat{n} \times \vec{S}_1 \cdot \vec{a}_1 \vec{v}_1 \cdot \vec{v}_1 \hat{n} \cdot \vec{v}_1 + \frac{7}{3} \hat{n} \times \vec{S}_1 \cdot \vec{v}_1 \vec{v}_1 \cdot \vec{v}_2 \hat{n} \cdot \vec{v}_1 + \\
& 3 \hat{n} \times \vec{S}_1 \cdot \vec{a}_1 \vec{v}_1 \cdot \vec{v}_2 \hat{n} \cdot \vec{v}_1 - \frac{9}{2} \hat{n} \times \vec{S}_1 \cdot \vec{v}_1 \vec{v}_2 \cdot \vec{a}_2 \hat{n} \cdot \vec{v}_1 - \frac{9}{4} \hat{n} \times \vec{S}_1 \cdot \vec{v}_1 \vec{v}_2 \cdot \vec{v}_2 \hat{n} \cdot \vec{v}_1 - \frac{3}{8} \hat{n} \times \vec{S}_1 \cdot \vec{a}_1 \vec{v}_2 \cdot \vec{v}_2 \hat{n} \cdot \vec{v}_1 + \\
& \frac{4}{3} \vec{S}_1 \times \vec{v}_1 \cdot \vec{a}_1 (\hat{n} \cdot \vec{v}_2)^2 + \frac{8}{3} \hat{n} \times \vec{S}_1 \cdot \vec{v}_1 \hat{n} \cdot \vec{a}_1 (\hat{n} \cdot \vec{v}_2)^2 - \frac{4}{3} \vec{S}_1 \times \vec{v}_1 \cdot \vec{v}_2 \hat{n} \cdot \vec{a}_1 \hat{n} \cdot \vec{v}_2 + \frac{2}{3} \vec{S}_1 \times \vec{v}_1 \cdot \vec{v}_2 \vec{a}_1 \cdot \vec{v}_2 - \\
& \frac{4}{3} \hat{n} \times \vec{S}_1 \cdot \vec{v}_1 \hat{n} \cdot \vec{v}_2 \vec{a}_1 \cdot \vec{v}_2 - \frac{11}{6} \vec{S}_1 \times \vec{v}_1 \cdot \vec{v}_2 \vec{v}_1 \cdot \vec{a}_1 + \frac{11}{3} \hat{n} \times \vec{S}_1 \cdot \vec{v}_1 \hat{n} \cdot \vec{v}_2 \vec{v}_1 \cdot \vec{a}_1 - \frac{25}{12} \vec{S}_1 \times \vec{v}_1 \cdot \vec{v}_2 \vec{v}_1 \cdot \vec{v}_1 - \\
& \frac{5}{2} \vec{S}_1 \times \vec{a}_1 \cdot \vec{v}_2 \vec{v}_1 \cdot \vec{v}_1 - \frac{1}{2} \vec{S}_1 \times \vec{v}_1 \cdot \vec{a}_1 \vec{v}_1 \cdot \vec{v}_1 - \frac{5}{6} \vec{S}_1 \times \vec{v}_1 \cdot \vec{a}_2 \vec{v}_1 \cdot \vec{v}_1 - \frac{11}{4} \hat{n} \times \vec{S}_1 \cdot \vec{v}_1 \hat{n} \cdot \vec{a}_1 \vec{v}_1 \cdot \vec{v}_1 + \\
& \frac{5}{3} \hat{n} \times \vec{S}_1 \cdot \vec{v}_1 \hat{n} \cdot \vec{a}_2 \vec{v}_1 \cdot \vec{v}_1 + \frac{25}{6} \hat{n} \times \vec{S}_1 \cdot \vec{v}_1 \hat{n} \cdot \vec{v}_2 \vec{v}_1 \cdot \vec{v}_1 + 5 \hat{n} \times \vec{S}_1 \cdot \vec{a}_1 \hat{n} \cdot \vec{v}_2 \vec{v}_1 \cdot \vec{v}_1 + \frac{13}{6} \vec{S}_1 \times \vec{v}_1 \cdot \vec{a}_1 \vec{v}_1 \cdot \vec{v}_2 + \\
& \frac{7}{6} \hat{n} \times \vec{S}_1 \cdot \vec{v}_1 \hat{n} \cdot \vec{a}_1 \vec{v}_1 \cdot \vec{v}_2 + \frac{1}{12} \vec{S}_1 \times \vec{v}_1 \cdot \vec{a}_1 \vec{v}_2 \cdot \vec{v}_2 - \frac{61}{24} \hat{n} \times \vec{S}_1 \cdot \vec{v}_1 \hat{n} \cdot \vec{a}_1 \vec{v}_2 \cdot \vec{v}_2 \Big) m_1 m_2 G^2 + \frac{1}{r^3} \\
& \Big( -2 \hat{n} \times \vec{S}_1 \cdot \vec{v}_1 (\hat{n} \cdot \vec{v}_1)^4 - \vec{S}_1 \times \vec{v}_1 \cdot \vec{v}_2 (\hat{n} \cdot \vec{v}_1)^3 + 6 \hat{n} \times \vec{S}_1 \cdot \vec{v}_1 \hat{n} \cdot \vec{v}_2 (\hat{n} \cdot \vec{v}_1)^3 - 4 \hat{n} \times \vec{S}_1 \cdot \vec{v}_1 (\hat{n} \cdot \vec{v}_2)^2 (\hat{n} \cdot \vec{v}_1)^2 + \\
& \frac{4}{3} \vec{S}_1 \times \vec{v}_1 \cdot \vec{v}_2 \hat{n} \cdot \vec{v}_2 (\hat{n} \cdot \vec{v}_1)^2 + \frac{15}{2} \hat{n} \times \vec{S}_1 \cdot \vec{v}_1 \vec{v}_1 \cdot \vec{v}_1 (\hat{n} \cdot \vec{v}_1)^2 - 3 \hat{n} \times \vec{S}_1 \cdot \vec{v}_1 \vec{v}_1 \cdot \vec{v}_2 (\hat{n} \cdot \vec{v}_1)^2 + \\
& \frac{53}{12} \hat{n} \times \vec{S}_1 \cdot \vec{v}_1 \vec{v}_2 \cdot \vec{v}_2 (\hat{n} \cdot \vec{v}_1)^2 + \frac{9}{2} \vec{S}_1 \times \vec{v}_1 \cdot \vec{v}_2 \vec{v}_1 \cdot \vec{v}_1 \hat{n} \cdot \vec{v}_1 - 18 \hat{n} \times \vec{S}_1 \cdot \vec{v}_1 \hat{n} \cdot \vec{v}_2 \vec{v}_1 \cdot \vec{v}_1 \hat{n} \cdot \vec{v}_1 - \\
& \frac{2}{3} \vec{S}_1 \times \vec{v}_1 \cdot \vec{v}_2 \vec{v}_1 \cdot \vec{v}_2 \hat{n} \cdot \vec{v}_1 + \frac{8}{3} \hat{n} \times \vec{S}_1 \cdot \vec{v}_1 \hat{n} \cdot \vec{v}_2 \vec{v}_1 \cdot \vec{v}_2 \hat{n} \cdot \vec{v}_1 + \frac{9}{4} \vec{S}_1 \times \vec{v}_1 \cdot \vec{v}_2 \vec{v}_2 \cdot \vec{v}_2 \hat{n} \cdot \vec{v}_1 - \\
& 9 \hat{n} \times \vec{S}_1 \cdot \vec{v}_1 \hat{n} \cdot \vec{v}_2 \vec{v}_2 \cdot \vec{v}_2 \hat{n} \cdot \vec{v}_1 - 2 \hat{n} \times \vec{S}_1 \cdot \vec{v}_1 (\vec{v}_1 \cdot \vec{v}_1)^2 - \frac{1}{3} \hat{n} \times \vec{S}_1 \cdot \vec{v}_1 (\vec{v}_1 \cdot \vec{v}_2)^2 + \\
& \frac{20}{3} \hat{n} \times \vec{S}_1 \cdot \vec{v}_1 (\hat{n} \cdot \vec{v}_2)^2 \vec{v}_1 \cdot \vec{v}_1 - \frac{10}{3} \vec{S}_1 \times \vec{v}_1 \cdot \vec{v}_2 \hat{n} \cdot \vec{v}_2 \vec{v}_1 \cdot \vec{v}_1 + \frac{9}{2} \hat{n} \times \vec{S}_1 \cdot \vec{v}_1 \vec{v}_1 \cdot \vec{v}_1 \vec{v}_1 \cdot \vec{v}_2 - \\
& \frac{19}{6} \hat{n} \times \vec{S}_1 \cdot \vec{v}_1 \vec{v}_1 \cdot \vec{v}_1 \vec{v}_2 \cdot \vec{v}_2 + \frac{9}{4} \hat{n} \times \vec{S}_1 \cdot \vec{v}_1 \vec{v}_1 \cdot \vec{v}_2 \vec{v}_2 \cdot \vec{v}_2 \Big) m_1 m_2 G^2 \Big\}
\end{aligned}$$

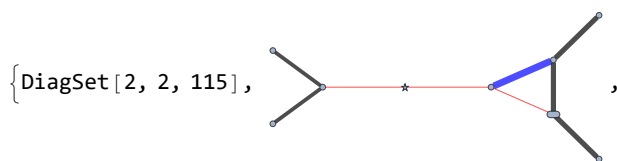

$$\frac{1}{r^2} G^2 m_1 m_2 \left( 2 (\hat{n} \cdot \vec{v}_1)^2 \vec{S}_1 \times \vec{a}_1 \cdot \vec{v}_2 - 8 \hat{n} \cdot \vec{v}_2 (\hat{n} \cdot \vec{v}_1)^2 \hat{n} \times \vec{S}_1 \cdot \vec{a}_1 + 4 \hat{n} \cdot \vec{a}_1 \hat{n} \cdot \vec{v}_1 \vec{S}_1 \times \vec{v}_1 \cdot \vec{v}_2 - \right. \\ \left. 16 \hat{n} \cdot \vec{a}_1 \hat{n} \cdot \vec{v}_2 \hat{n} \cdot \vec{v}_1 \hat{n} \times \vec{S}_1 \cdot \vec{v}_1 + 4 \vec{a}_1 \cdot \vec{v}_2 \hat{n} \cdot \vec{v}_1 \hat{n} \times \vec{S}_1 \cdot \vec{v}_1 + 4 \vec{v}_1 \cdot \vec{v}_2 \hat{n} \cdot \vec{v}_1 \hat{n} \times \vec{S}_1 \cdot \vec{a}_1 + 4 \vec{v}_1 \cdot \vec{a}_1 \hat{n} \cdot \vec{v}_2 \hat{n} \times \vec{S}_1 \cdot \vec{v}_1 + \right. \\ \left. 2 \vec{v}_1 \cdot \vec{v}_1 \hat{n} \cdot \vec{v}_2 \hat{n} \times \vec{S}_1 \cdot \vec{a}_1 + 4 \vec{v}_1 \cdot \vec{v}_2 \hat{n} \cdot \vec{a}_1 \hat{n} \times \vec{S}_1 \cdot \vec{v}_1 - 2 \vec{v}_1 \cdot \vec{a}_1 \vec{S}_1 \times \vec{v}_1 \cdot \vec{v}_2 - \vec{v}_1 \cdot \vec{v}_1 \vec{S}_1 \times \vec{a}_1 \cdot \vec{v}_2 + 2 (\hat{n} \cdot \vec{v}_1)^2 \right. \\ \left. \frac{1}{\vec{S}_1 \times \vec{v}_1 \cdot \vec{v}_2} - 8 \hat{n} \cdot \vec{v}_2 (\hat{n} \cdot \vec{v}_1)^2 \hat{n} \times \frac{1}{\vec{S}_1 \cdot \vec{v}_1} + 4 \vec{v}_1 \cdot \vec{v}_2 \hat{n} \cdot \vec{v}_1 \hat{n} \times \frac{1}{\vec{S}_1 \cdot \vec{v}_1} + 2 \vec{v}_1 \cdot \vec{v}_1 \hat{n} \cdot \vec{v}_2 \hat{n} \times \frac{1}{\vec{S}_1 \cdot \vec{v}_1} - \vec{v}_1 \cdot \vec{v}_1 \frac{1}{\vec{S}_1 \times \vec{v}_1 \cdot \vec{v}_2} \right) + \\ \frac{1}{r^3} G^2 m_1 m_2 \left( -8 (\hat{n} \cdot \vec{v}_1)^3 \vec{S}_1 \times \vec{v}_1 \cdot \vec{v}_2 + 48 \hat{n} \cdot \vec{v}_2 (\hat{n} \cdot \vec{v}_1)^3 \hat{n} \times \vec{S}_1 \cdot \vec{v}_1 - 24 \vec{v}_1 \cdot \vec{v}_2 (\hat{n} \cdot \vec{v}_1)^2 \hat{n} \times \vec{S}_1 \cdot \vec{v}_1 + \right. \\ \left. 6 \vec{v}_1 \cdot \vec{v}_1 \hat{n} \cdot \vec{v}_1 \vec{S}_1 \times \vec{v}_1 \cdot \vec{v}_2 - 24 \vec{v}_1 \cdot \vec{v}_1 \hat{n} \cdot \vec{v}_2 \hat{n} \cdot \vec{v}_1 \hat{n} \times \vec{S}_1 \cdot \vec{v}_1 + 6 \vec{v}_1 \cdot \vec{v}_1 \vec{v}_1 \cdot \vec{v}_2 \hat{n} \times \vec{S}_1 \cdot \vec{v}_1 \right) \Big\}$$

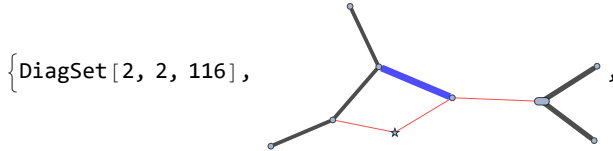

$$\frac{1}{r^2} G^2 \left( -\frac{16}{3} \hat{n} \times \vec{S}_1 \cdot \vec{v}_1 (\hat{n} \cdot \vec{v}_2)^3 + \frac{16}{3} \hat{n} \times \vec{a}_1 \cdot \vec{S}_1 (\hat{n} \cdot \vec{v}_2)^3 + 4 \vec{S}_1 \times \vec{v}_1 \cdot \vec{v}_2 (\hat{n} \cdot \vec{v}_2)^2 - 4 \vec{a}_1 \times \vec{S}_1 \cdot \vec{v}_2 (\hat{n} \cdot \vec{v}_2)^2 + \right. \\ \left. \frac{8}{3} \vec{a}_2 \times \vec{S}_1 \cdot \vec{v}_1 (\hat{n} \cdot \vec{v}_2)^2 - \frac{32}{3} \hat{n} \times \vec{S}_1 \cdot \vec{v}_1 \hat{n} \cdot \vec{a}_2 (\hat{n} \cdot \vec{v}_2)^2 + \frac{16}{3} \vec{S}_1 \times \vec{v}_1 \cdot \vec{v}_2 \hat{n} \cdot \vec{a}_2 \hat{n} \cdot \vec{v}_2 + \right. \\ \left. \frac{28}{3} \hat{n} \times \vec{S}_1 \cdot \vec{v}_1 \vec{a}_2 \cdot \vec{v}_2 \hat{n} \cdot \vec{v}_2 + 8 \hat{n} \times \vec{S}_1 \cdot \vec{v}_1 \vec{v}_2 \cdot \vec{v}_2 \hat{n} \cdot \vec{v}_2 - 8 \hat{n} \times \vec{a}_1 \cdot \vec{S}_1 \vec{v}_2 \cdot \vec{v}_2 \hat{n} \cdot \vec{v}_2 - \frac{14}{3} \vec{S}_1 \times \vec{v}_1 \cdot \vec{v}_2 \vec{a}_2 \cdot \vec{v}_2 - \right. \\ \left. 4 \vec{S}_1 \times \vec{v}_1 \cdot \vec{v}_2 \vec{v}_2 \cdot \vec{v}_2 + 4 \vec{a}_1 \times \vec{S}_1 \cdot \vec{v}_2 \vec{v}_2 \cdot \vec{v}_2 - \frac{10}{3} \vec{a}_2 \times \vec{S}_1 \cdot \vec{v}_1 \vec{v}_2 \cdot \vec{v}_2 + \frac{20}{3} \hat{n} \times \vec{S}_1 \cdot \vec{v}_1 \hat{n} \cdot \vec{a}_2 \vec{v}_2 \cdot \vec{v}_2 \right) m_2^2 + \frac{1}{r^3} \\ G^2 \left( -8 \hat{n} \times \vec{S}_1 \cdot \vec{v}_1 (\hat{n} \cdot \vec{v}_2)^4 + \frac{16}{3} \vec{S}_1 \times \vec{v}_1 \cdot \vec{v}_2 (\hat{n} \cdot \vec{v}_2)^3 + 32 \hat{n} \times \vec{S}_1 \cdot \vec{v}_1 \hat{n} \cdot \vec{v}_1 (\hat{n} \cdot \vec{v}_2)^3 - 16 \vec{S}_1 \times \vec{v}_1 \cdot \vec{v}_2 \hat{n} \cdot \vec{v}_1 (\hat{n} \cdot \vec{v}_2)^2 - \right. \\ \left. 16 \hat{n} \times \vec{S}_1 \cdot \vec{v}_1 \vec{v}_1 \cdot \vec{v}_2 (\hat{n} \cdot \vec{v}_2)^2 + 12 \hat{n} \times \vec{S}_1 \cdot \vec{v}_1 \vec{v}_2 \cdot \vec{v}_2 (\hat{n} \cdot \vec{v}_2)^2 + 8 \vec{S}_1 \times \vec{v}_1 \cdot \vec{v}_2 \vec{v}_1 \cdot \vec{v}_2 \hat{n} \cdot \vec{v}_2 - 6 \vec{S}_1 \times \vec{v}_1 \cdot \vec{v}_2 \vec{v}_2 \cdot \vec{v}_2 \hat{n} \cdot \vec{v}_2 - \right. \\ \left. 32 \hat{n} \times \vec{S}_1 \cdot \vec{v}_1 \hat{n} \cdot \vec{v}_1 \vec{v}_2 \cdot \vec{v}_2 \hat{n} \cdot \vec{v}_2 - 2 \hat{n} \times \vec{S}_1 \cdot \vec{v}_1 (\vec{v}_2 \cdot \vec{v}_2)^2 + 8 \vec{S}_1 \times \vec{v}_1 \cdot \vec{v}_2 \hat{n} \cdot \vec{v}_1 \vec{v}_2 \cdot \vec{v}_2 + 8 \hat{n} \times \vec{S}_1 \cdot \vec{v}_1 \vec{v}_1 \cdot \vec{v}_2 \vec{v}_2 \cdot \vec{v}_2 \right) m_2^2 \Big\}$$

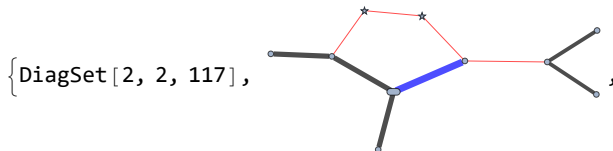

$$\frac{1}{r} \left( -\frac{7}{48} \hat{n} \times \vec{S}_1 \cdot \vec{v}_1 (\hat{n} \cdot \vec{a}_1)^2 + \frac{1}{12} \vec{S}_1 \times \vec{v}_1 \cdot \vec{v}_2 \hat{n} \cdot \vec{a}_1 - \frac{1}{8} \vec{S}_1 \times \vec{v}_1 \cdot \vec{a}_1 \hat{n} \cdot \vec{a}_1 + \frac{1}{24} \vec{S}_1 \times \vec{v}_1 \cdot \vec{a}_2 \hat{n} \cdot \vec{a}_1 - \right. \\ \left. \frac{1}{12} \hat{n} \times \vec{S}_1 \cdot \vec{v}_1 \hat{n} \cdot \vec{a}_2 \hat{n} \cdot \vec{a}_1 + \frac{1}{3} \hat{n} \times \vec{S}_1 \cdot \vec{v}_1 \hat{n} \cdot \vec{v}_1 \hat{n} \cdot \vec{a}_1 - \frac{13}{24} \hat{n} \times \vec{S}_1 \cdot \vec{a}_1 \hat{n} \cdot \vec{v}_1 \hat{n} \cdot \vec{a}_1 - \frac{1}{6} \hat{n} \times \vec{S}_1 \cdot \vec{v}_1 \hat{n} \cdot \vec{v}_2 \hat{n} \cdot \vec{a}_1 - \right. \\ \left. \frac{1}{3} \hat{n} \times \vec{S}_1 \cdot \vec{a}_1 (\hat{n} \cdot \vec{v}_1)^2 + \frac{11}{48} \hat{n} \times \vec{S}_1 \cdot \vec{v}_1 (\hat{n} \cdot \vec{v}_1)^2 + \frac{1}{48} \hat{n} \times \vec{S}_1 \cdot \vec{a}_1 (\hat{n} \cdot \vec{v}_1)^2 + \frac{1}{12} \vec{S}_1 \times \vec{v}_1 \cdot \vec{a}_1 \hat{n} \cdot \vec{a}_2 - \right. \\ \left. \frac{1}{12} \vec{S}_1 \times \vec{a}_1 \cdot \vec{v}_2 \hat{n} \cdot \vec{v}_1 - \frac{1}{2} \vec{S}_1 \times \vec{v}_1 \cdot \vec{a}_1 \hat{n} \cdot \vec{v}_1 - \frac{1}{24} \vec{S}_1 \times \vec{a}_1 \cdot \vec{a}_2 \hat{n} \cdot \vec{v}_1 - \frac{1}{12} \vec{S}_1 \times \vec{v}_1 \cdot \vec{a}_1 \hat{n} \cdot \vec{v}_1 + \frac{5}{24} \hat{n} \times \vec{S}_1 \cdot \vec{v}_1 \hat{n} \cdot \vec{a}_1 \hat{n} \cdot \vec{v}_1 + \right. \\ \left. \frac{1}{12} \hat{n} \times \vec{S}_1 \cdot \vec{a}_1 \hat{n} \cdot \vec{a}_2 \hat{n} \cdot \vec{v}_1 + \frac{1}{6} \vec{S}_1 \times \vec{v}_1 \cdot \vec{a}_1 \hat{n} \cdot \vec{v}_2 + \frac{1}{6} \hat{n} \times \vec{S}_1 \cdot \vec{a}_1 \hat{n} \cdot \vec{v}_1 \hat{n} \cdot \vec{v}_2 + \frac{17}{48} \hat{n} \times \vec{S}_1 \cdot \vec{v}_1 \vec{a}_1 \cdot \vec{a}_1 + \right. \\ \left. \frac{1}{24} \hat{n} \times \vec{S}_1 \cdot \vec{v}_1 \vec{a}_1 \cdot \vec{a}_2 + \frac{1}{12} \hat{n} \times \vec{S}_1 \cdot \vec{v}_1 \vec{a}_1 \cdot \vec{v}_2 - \frac{7}{24} \hat{n} \times \vec{S}_1 \cdot \vec{v}_1 \vec{v}_1 \cdot \vec{a}_1 - \frac{1}{6} \hat{n} \times \vec{S}_1 \cdot \vec{v}_1 \vec{v}_1 \cdot \vec{a}_1 + \frac{5}{6} \hat{n} \times \vec{S}_1 \cdot \vec{a}_1 \vec{v}_1 \cdot \vec{a}_1 - \right. \\ \left. \frac{1}{24} \hat{n} \times \vec{S}_1 \cdot \vec{a}_1 \vec{v}_1 \cdot \vec{a}_2 + \frac{1}{6} \hat{n} \times \vec{S}_1 \cdot \vec{a}_1 \vec{v}_1 \cdot \vec{v}_1 - \frac{19}{48} \hat{n} \times \vec{S}_1 \cdot \vec{v}_1 \vec{v}_1 \cdot \vec{v}_1 - \frac{5}{48} \hat{n} \times \vec{S}_1 \cdot \vec{a}_1 \vec{v}_1 \cdot \vec{v}_1 - \frac{1}{12} \hat{n} \times \vec{S}_1 \cdot \vec{a}_1 \vec{v}_1 \cdot \vec{v}_2 \right) m_1 m_2 \\ G^2 + \frac{1}{r^2} \left( -\left( \hat{n} \times \vec{S}_1 \cdot \vec{v}_1 \right) (\hat{n} \cdot \vec{v}_1)^3 + \frac{13}{12} \hat{n} \times \vec{S}_1 \cdot \vec{a}_1 (\hat{n} \cdot \vec{v}_1)^3 - \frac{11}{24} \vec{S}_1 \times \vec{v}_1 \cdot \vec{v}_2 (\hat{n} \cdot \vec{v}_1)^2 + \frac{1}{3} \vec{S}_1 \times \vec{a}_1 \cdot \vec{v}_2 (\hat{n} \cdot \vec{v}_1)^2 + \right. \\ \left. \frac{53}{48} \vec{S}_1 \times \vec{v}_1 \cdot \vec{a}_1 (\hat{n} \cdot \vec{v}_1)^2 - \frac{11}{48} \vec{S}_1 \times \vec{v}_1 \cdot \vec{a}_2 (\hat{n} \cdot \vec{v}_1)^2 - \frac{7}{6} \hat{n} \times \vec{S}_1 \cdot \vec{v}_1 \hat{n} \cdot \vec{a}_1 (\hat{n} \cdot \vec{v}_1)^2 + \frac{11}{12} \hat{n} \times \vec{S}_1 \cdot \vec{v}_1 \hat{n} \cdot \vec{a}_2 (\hat{n} \cdot \vec{v}_1)^2 + \right.$$

$$\begin{aligned}
 & \frac{11}{6} \hat{n} \times \vec{S}_1 \cdot \vec{v}_1 \hat{n} \cdot \vec{v}_2 (\hat{n} \cdot \vec{v}_1)^2 - \frac{4}{3} \hat{n} \times \vec{S}_1 \cdot \vec{a}_1 \hat{n} \cdot \vec{v}_2 (\hat{n} \cdot \vec{v}_1)^2 + \frac{1}{3} \hat{n} \times \vec{S}_1 \cdot \vec{a}_1 (\hat{n} \cdot \vec{v}_2)^2 \hat{n} \cdot \vec{v}_1 - \\
 & \frac{1}{3} \vec{S}_1 \times \vec{v}_1 \cdot \vec{v}_2 \hat{n} \cdot \vec{a}_1 \hat{n} \cdot \vec{v}_1 - \frac{1}{6} \vec{S}_1 \times \vec{a}_1 \cdot \vec{v}_2 \hat{n} \cdot \vec{v}_2 \hat{n} \cdot \vec{v}_1 - \vec{S}_1 \times \vec{v}_1 \cdot \vec{a}_1 \hat{n} \cdot \vec{v}_2 \hat{n} \cdot \vec{v}_1 + \frac{4}{3} \hat{n} \times \vec{S}_1 \cdot \vec{v}_1 \hat{n} \cdot \vec{a}_1 \hat{n} \cdot \vec{v}_2 \hat{n} \cdot \vec{v}_1 - \\
 & \frac{1}{3} \hat{n} \times \vec{S}_1 \cdot \vec{v}_1 \vec{a}_1 \cdot \vec{v}_2 \hat{n} \cdot \vec{v}_1 + \frac{5}{24} \hat{n} \times \vec{S}_1 \cdot \vec{v}_1 \vec{v}_1 \cdot \vec{a}_1 \hat{n} \cdot \vec{v}_1 - \frac{11}{24} \hat{n} \times \vec{S}_1 \cdot \vec{v}_1 \vec{v}_1 \cdot \vec{a}_2 \hat{n} \cdot \vec{v}_1 - \hat{n} \times \vec{S}_1 \cdot \vec{a}_1 \vec{v}_1 \cdot \vec{v}_1 \hat{n} \cdot \vec{v}_1 - \\
 & \frac{11}{12} \hat{n} \times \vec{S}_1 \cdot \vec{v}_1 \vec{v}_1 \cdot \vec{v}_2 \hat{n} \cdot \vec{v}_1 + \frac{2}{3} \hat{n} \times \vec{S}_1 \cdot \vec{a}_1 \vec{v}_1 \cdot \vec{v}_2 \hat{n} \cdot \vec{v}_1 - \frac{1}{12} \hat{n} \times \vec{S}_1 \cdot \vec{a}_1 \vec{v}_2 \cdot \vec{v}_2 \hat{n} \cdot \vec{v}_1 + \frac{1}{6} \vec{S}_1 \times \vec{v}_1 \cdot \vec{a}_1 (\hat{n} \cdot \vec{v}_2)^2 - \\
 & \frac{1}{3} \hat{n} \times \vec{S}_1 \cdot \vec{v}_1 \hat{n} \cdot \vec{a}_1 (\hat{n} \cdot \vec{v}_2)^2 + \frac{1}{6} \vec{S}_1 \times \vec{v}_1 \cdot \vec{v}_2 \hat{n} \cdot \vec{a}_1 \hat{n} \cdot \vec{v}_2 - \frac{1}{12} \vec{S}_1 \times \vec{v}_1 \cdot \vec{v}_2 \vec{a}_1 \cdot \vec{v}_2 + \frac{1}{6} \hat{n} \times \vec{S}_1 \cdot \vec{v}_1 \hat{n} \cdot \vec{v}_2 \vec{a}_1 \cdot \vec{v}_2 + \\
 & \frac{1}{6} \vec{S}_1 \times \vec{v}_1 \cdot \vec{v}_2 \vec{v}_1 \cdot \vec{a}_1 - \frac{1}{3} \hat{n} \times \vec{S}_1 \cdot \vec{v}_1 \hat{n} \cdot \vec{v}_2 \vec{v}_1 \cdot \vec{a}_1 + \frac{19}{24} \vec{S}_1 \times \vec{v}_1 \cdot \vec{v}_2 \vec{v}_1 \cdot \vec{v}_1 - \frac{1}{6} \vec{S}_1 \times \vec{a}_1 \cdot \vec{v}_2 \vec{v}_1 \cdot \vec{v}_1 - \\
 & \frac{13}{48} \vec{S}_1 \times \vec{v}_1 \cdot \vec{a}_1 \vec{v}_1 \cdot \vec{v}_1 + \frac{19}{48} \vec{S}_1 \times \vec{v}_1 \cdot \vec{a}_2 \vec{v}_1 \cdot \vec{v}_1 - \frac{11}{24} \hat{n} \times \vec{S}_1 \cdot \vec{v}_1 \hat{n} \cdot \vec{a}_1 \vec{v}_1 \cdot \vec{v}_1 - \frac{19}{24} \hat{n} \times \vec{S}_1 \cdot \vec{v}_1 \hat{n} \cdot \vec{a}_2 \vec{v}_1 \cdot \vec{v}_1 - \\
 & \frac{19}{12} \hat{n} \times \vec{S}_1 \cdot \vec{v}_1 \hat{n} \cdot \vec{v}_2 \vec{v}_1 \cdot \vec{v}_1 + \frac{1}{3} \hat{n} \times \vec{S}_1 \cdot \vec{a}_1 \hat{n} \cdot \vec{v}_2 \vec{v}_1 \cdot \vec{v}_1 + \frac{1}{12} \vec{S}_1 \times \vec{a}_1 \cdot \vec{v}_2 \vec{v}_1 \cdot \vec{v}_2 + \frac{1}{2} \vec{S}_1 \times \vec{v}_1 \cdot \vec{a}_1 \vec{v}_1 \cdot \vec{v}_2 - \\
 & \frac{1}{3} \hat{n} \times \vec{S}_1 \cdot \vec{v}_1 \hat{n} \cdot \vec{a}_1 \vec{v}_1 \cdot \vec{v}_2 - \frac{1}{6} \hat{n} \times \vec{S}_1 \cdot \vec{a}_1 \hat{n} \cdot \vec{v}_2 \vec{v}_1 \cdot \vec{v}_2 - \frac{1}{12} \vec{S}_1 \times \vec{v}_1 \cdot \vec{a}_1 \vec{v}_2 \cdot \vec{v}_2 + \frac{1}{12} \hat{n} \times \vec{S}_1 \cdot \vec{v}_1 \hat{n} \cdot \vec{a}_1 \vec{v}_2 \cdot \vec{v}_2 \Big) m_1 m_2 G^2 + \\
 & \frac{1}{r^3} \left( \frac{73}{32} \hat{n} \times \vec{S}_1 \cdot \vec{v}_1 (\hat{n} \cdot \vec{v}_1)^4 + \vec{S}_1 \times \vec{v}_1 \cdot \vec{v}_2 (\hat{n} \cdot \vec{v}_1)^3 - 6 \hat{n} \times \vec{S}_1 \cdot \vec{v}_1 \hat{n} \cdot \vec{v}_2 (\hat{n} \cdot \vec{v}_1)^3 + \right. \\
 & \frac{11}{2} \hat{n} \times \vec{S}_1 \cdot \vec{v}_1 (\hat{n} \cdot \vec{v}_2)^2 (\hat{n} \cdot \vec{v}_1)^2 - \frac{11}{6} \vec{S}_1 \times \vec{v}_1 \cdot \vec{v}_2 \hat{n} \cdot \vec{v}_2 (\hat{n} \cdot \vec{v}_1)^2 + \frac{1}{16} \hat{n} \times \vec{S}_1 \cdot \vec{v}_1 \vec{v}_1 \cdot \vec{v}_1 (\hat{n} \cdot \vec{v}_1)^2 + \\
 & 3 \hat{n} \times \vec{S}_1 \cdot \vec{v}_1 \vec{v}_1 \cdot \vec{v}_2 (\hat{n} \cdot \vec{v}_1)^2 - \frac{11}{12} \hat{n} \times \vec{S}_1 \cdot \vec{v}_1 \vec{v}_2 \cdot \vec{v}_2 (\hat{n} \cdot \vec{v}_1)^2 + \frac{11}{12} \vec{S}_1 \times \vec{v}_1 \cdot \vec{v}_2 \vec{v}_1 \cdot \vec{v}_2 \hat{n} \cdot \vec{v}_1 - \\
 & \frac{11}{3} \hat{n} \times \vec{S}_1 \cdot \vec{v}_1 \hat{n} \cdot \vec{v}_2 \vec{v}_1 \cdot \vec{v}_2 \hat{n} \cdot \vec{v}_1 - \frac{19}{32} \hat{n} \times \vec{S}_1 \cdot \vec{v}_1 (\vec{v}_1 \cdot \vec{v}_1)^2 + \frac{11}{24} \hat{n} \times \vec{S}_1 \cdot \vec{v}_1 (\vec{v}_1 \cdot \vec{v}_2)^2 - \\
 & \left. \frac{19}{6} \hat{n} \times \vec{S}_1 \cdot \vec{v}_1 (\hat{n} \cdot \vec{v}_2)^2 \vec{v}_1 \cdot \vec{v}_1 + \frac{19}{12} \vec{S}_1 \times \vec{v}_1 \cdot \vec{v}_2 \hat{n} \cdot \vec{v}_2 \vec{v}_1 \cdot \vec{v}_1 + \frac{19}{24} \hat{n} \times \vec{S}_1 \cdot \vec{v}_1 \vec{v}_1 \cdot \vec{v}_1 \vec{v}_2 \cdot \vec{v}_2 \right) m_1 m_2 G^2 + \\
 & m_1 m_2 \left( -\frac{1}{12} \log \left( \frac{r}{R_\theta} \right) \vec{S}_1 \times \vec{v}_1 \cdot \vec{a}_1 + \frac{17}{144} \vec{S}_1 \times \vec{v}_1 \cdot \vec{a}_1 - \frac{17}{144} \vec{S}_1 \times \vec{a}_1 \cdot \vec{a}_1 + \frac{1}{24} \hat{n} \times \vec{S}_1 \cdot \vec{a}_1 \hat{n} \cdot \vec{a}_1 - \frac{1}{24} \hat{n} \times \vec{S}_1 \cdot \vec{v}_1 \hat{n} \cdot \vec{a}_1 - \right. \\
 & \left. \frac{1}{24} \hat{n} \times \vec{S}_1 \cdot \vec{a}_1 \hat{n} \cdot \vec{a}_1 + \frac{1}{24} \hat{n} \times \vec{S}_1 \cdot \vec{a}_1 \hat{n} \cdot \vec{v}_1 + \frac{1}{12} \vec{S}_1 \times \vec{a}_1 \cdot \vec{a}_1 \log \left( \frac{r}{R_\theta} \right) + \frac{\frac{1}{24} \vec{S}_1 \times \vec{v}_1 \cdot \vec{a}_1 - \frac{1}{24} \vec{S}_1 \times \vec{a}_1 \cdot \vec{a}_1}{\epsilon_d} \right) G^2 \Big\}
 \end{aligned}$$

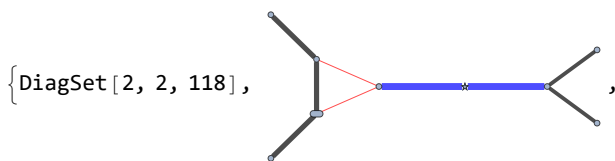

$$\begin{aligned}
 & \frac{1}{r} \left( -\frac{1}{3} \vec{S}_1 \times \vec{v}_1 \cdot \vec{v}_2 \hat{n} \cdot \vec{a}_2 - \frac{1}{3} \vec{S}_1 \times \vec{a}_1 \cdot \vec{v}_2 \hat{n} \cdot \vec{a}_2 + \frac{2}{3} \hat{n} \times \vec{S}_1 \cdot \vec{v}_1 \hat{n} \cdot \vec{v}_2 \hat{n} \cdot \vec{a}_2 + \frac{2}{3} \hat{n} \times \vec{S}_1 \cdot \vec{a}_1 \hat{n} \cdot \vec{v}_2 \hat{n} \cdot \vec{a}_2 - \right. \\
 & \left. \frac{1}{3} \vec{S}_1 \times \vec{v}_1 \cdot \vec{a}_2 \hat{n} \cdot \vec{v}_2 - \frac{1}{3} \vec{S}_1 \times \vec{a}_1 \cdot \vec{a}_2 \hat{n} \cdot \vec{v}_2 - \frac{4}{3} \hat{n} \times \vec{S}_1 \cdot \vec{v}_1 \vec{v}_2 \cdot \vec{a}_2 - \frac{4}{3} \hat{n} \times \vec{S}_1 \cdot \vec{a}_1 \vec{v}_2 \cdot \vec{a}_2 \right) m_1 m_2 G^2 + \\
 & \frac{1}{r^2} \left( \frac{4}{3} \hat{n} \times \vec{S}_1 \cdot \vec{v}_1 (\hat{n} \cdot \vec{v}_2)^3 + \frac{4}{3} \hat{n} \times \vec{S}_1 \cdot \vec{a}_1 (\hat{n} \cdot \vec{v}_2)^3 - \vec{S}_1 \times \vec{v}_1 \cdot \vec{v}_2 (\hat{n} \cdot \vec{v}_2)^2 - \vec{S}_1 \times \vec{a}_1 \cdot \vec{v}_2 (\hat{n} \cdot \vec{v}_2)^2 + \right. \\
 & \frac{2}{3} \vec{S}_1 \times \vec{v}_1 \cdot \vec{a}_2 \hat{n} \cdot \vec{v}_1 \hat{n} \cdot \vec{v}_2 - \frac{8}{3} \hat{n} \times \vec{S}_1 \cdot \vec{v}_1 \hat{n} \cdot \vec{a}_2 \hat{n} \cdot \vec{v}_1 \hat{n} \cdot \vec{v}_2 + \frac{2}{3} \hat{n} \times \vec{S}_1 \cdot \vec{v}_1 \vec{v}_1 \cdot \vec{a}_2 \hat{n} \cdot \vec{v}_2 - 2 \hat{n} \times \vec{S}_1 \cdot \vec{v}_1 \vec{v}_2 \cdot \vec{v}_2 \hat{n} \cdot \vec{v}_2 - \\
 & 2 \hat{n} \times \vec{S}_1 \cdot \vec{a}_1 \vec{v}_2 \cdot \vec{v}_2 \hat{n} \cdot \vec{v}_2 + \frac{2}{3} \vec{S}_1 \times \vec{v}_1 \cdot \vec{v}_2 \hat{n} \cdot \vec{a}_2 \hat{n} \cdot \vec{v}_1 - \frac{1}{3} \vec{S}_1 \times \vec{v}_1 \cdot \vec{v}_2 \vec{v}_1 \cdot \vec{a}_2 - \frac{1}{3} \vec{S}_1 \times \vec{v}_1 \cdot \vec{a}_2 \vec{v}_1 \cdot \vec{v}_2 + \\
 & \left. \frac{2}{3} \hat{n} \times \vec{S}_1 \cdot \vec{v}_1 \hat{n} \cdot \vec{a}_2 \vec{v}_1 \cdot \vec{v}_2 + \frac{8}{3} \hat{n} \times \vec{S}_1 \cdot \vec{v}_1 \hat{n} \cdot \vec{v}_1 \vec{v}_2 \cdot \vec{a}_2 + \vec{S}_1 \times \vec{v}_1 \cdot \vec{v}_2 \vec{v}_2 \cdot \vec{v}_2 + \vec{S}_1 \times \vec{a}_1 \cdot \vec{v}_2 \vec{v}_2 \cdot \vec{v}_2 \right) m_1 m_2 G^2 + \frac{1}{r^3}
 \end{aligned}$$

$$\left( -8 \hat{n} \times \vec{S}_1 \cdot \vec{v}_1 \hat{n} \cdot \vec{v}_1 (\hat{n} \cdot \vec{v}_2)^3 + 4 \vec{S}_1 \times \vec{v}_1 \cdot \vec{v}_2 \hat{n} \cdot \vec{v}_1 (\hat{n} \cdot \vec{v}_2)^2 + 4 \hat{n} \times \vec{S}_1 \cdot \vec{v}_1 \vec{v}_1 \cdot \vec{v}_2 (\hat{n} \cdot \vec{v}_2)^2 - 2 \vec{S}_1 \times \vec{v}_1 \cdot \vec{v}_2 \vec{v}_1 \cdot \vec{v}_2 \hat{n} \cdot \vec{v}_2 + 8 \hat{n} \times \vec{S}_1 \cdot \vec{v}_1 \hat{n} \cdot \vec{v}_1 \vec{v}_2 \cdot \vec{v}_2 \hat{n} \cdot \vec{v}_2 - 2 \vec{S}_1 \times \vec{v}_1 \cdot \vec{v}_2 \hat{n} \cdot \vec{v}_1 \vec{v}_2 \cdot \vec{v}_2 - 2 \hat{n} \times \vec{S}_1 \cdot \vec{v}_1 \vec{v}_1 \cdot \vec{v}_2 \vec{v}_2 \cdot \vec{v}_2 \right) m_1 m_2 G^2 \}$$

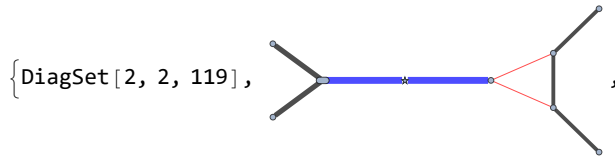

$$\begin{aligned} & \frac{1}{r} G^2 \left( \frac{1}{12} \vec{S}_1 \times \vec{v}_1 \cdot \vec{v}_2 \hat{n} \cdot \vec{a}_1 - \frac{1}{6} \hat{n} \times \vec{S}_1 \cdot \vec{v}_1 \hat{n} \cdot \vec{v}_2 \hat{n} \cdot \vec{a}_1 + \frac{5}{24} \vec{S}_1 \times \vec{v}_1 \cdot \vec{v}_2 \hat{n} \cdot \vec{a}_1 - \frac{1}{4} \vec{a}_1 \times \vec{S}_1 \cdot \vec{v}_2 \hat{n} \cdot \vec{a}_1 + \right. \\ & \frac{1}{6} \vec{S}_1 \times \vec{v}_1 \cdot \vec{v}_2 \hat{n} \cdot \vec{a}_2 - \frac{1}{6} \vec{a}_1 \times \vec{S}_1 \cdot \vec{v}_2 \hat{n} \cdot \vec{a}_2 - \frac{1}{6} \vec{a}_1 \times \vec{S}_1 \cdot \vec{v}_2 \hat{n} \cdot \vec{v}_1 + \frac{1}{8} \vec{S}_1 \times \vec{v}_1 \cdot \vec{v}_2 \hat{n} \cdot \vec{v}_1 - \\ & \frac{7}{24} \vec{a}_1 \times \vec{S}_1 \cdot \vec{v}_2 \hat{n} \cdot \vec{v}_1 - \frac{1}{3} \vec{a}_1 \times \vec{S}_1 \cdot \vec{v}_1 \hat{n} \cdot \vec{v}_2 - \frac{1}{3} \vec{a}_1 \times \vec{S}_1 \cdot \vec{v}_1 \hat{n} \cdot \vec{v}_2 + \frac{1}{6} \vec{a}_1 \times \vec{a}_2 \cdot \vec{S}_1 \hat{n} \cdot \vec{v}_2 + \\ & \frac{1}{6} \vec{a}_2 \times \vec{S}_1 \cdot \vec{v}_1 \hat{n} \cdot \vec{v}_2 - \frac{5}{12} \hat{n} \times \vec{S}_1 \cdot \vec{v}_1 \hat{n} \cdot \vec{a}_1 \hat{n} \cdot \vec{v}_2 + \frac{1}{2} \hat{n} \times \vec{a}_1 \cdot \vec{S}_1 \hat{n} \cdot \vec{a}_1 \hat{n} \cdot \vec{v}_2 - \frac{1}{3} \hat{n} \times \vec{S}_1 \cdot \vec{v}_1 \hat{n} \cdot \vec{a}_2 \hat{n} \cdot \vec{v}_2 + \\ & \frac{1}{3} \hat{n} \times \vec{a}_1 \cdot \vec{S}_1 \hat{n} \cdot \vec{a}_2 \hat{n} \cdot \vec{v}_2 + \frac{1}{3} \hat{n} \times \vec{a}_1 \cdot \vec{S}_1 \hat{n} \cdot \vec{v}_1 \hat{n} \cdot \vec{v}_2 - \frac{1}{4} \hat{n} \times \vec{S}_1 \cdot \vec{v}_1 \hat{n} \cdot \vec{v}_1 \hat{n} \cdot \vec{v}_2 + \frac{7}{12} \hat{n} \times \vec{a}_1 \cdot \vec{S}_1 \hat{n} \cdot \vec{v}_1 \hat{n} \cdot \vec{v}_2 + \\ & \frac{1}{12} \hat{n} \times \vec{S}_1 \cdot \vec{v}_1 \vec{a}_1 \cdot \vec{v}_2 + \frac{5}{24} \hat{n} \times \vec{S}_1 \cdot \vec{v}_1 \vec{a}_1 \cdot \vec{v}_2 - \frac{1}{4} \hat{n} \times \vec{a}_1 \cdot \vec{S}_1 \vec{a}_1 \cdot \vec{v}_2 - \frac{5}{6} \hat{n} \times \vec{S}_1 \cdot \vec{v}_1 \vec{a}_2 \cdot \vec{v}_2 + \\ & \left. \frac{5}{6} \hat{n} \times \vec{a}_1 \cdot \vec{S}_1 \vec{a}_2 \cdot \vec{v}_2 - \frac{1}{6} \hat{n} \times \vec{a}_1 \cdot \vec{S}_1 \vec{v}_1 \cdot \vec{v}_2 + \frac{1}{8} \hat{n} \times \vec{S}_1 \cdot \vec{v}_1 \vec{v}_1 \cdot \vec{v}_2 - \frac{7}{24} \hat{n} \times \vec{a}_1 \cdot \vec{S}_1 \vec{v}_1 \cdot \vec{v}_2 \right) m_2^2 + \frac{1}{r^2} \\ & G^2 \left( -\frac{2}{3} \hat{n} \times \vec{S}_1 \cdot \vec{v}_1 (\hat{n} \cdot \vec{v}_2)^3 + \frac{2}{3} \hat{n} \times \vec{a}_1 \cdot \vec{S}_1 (\hat{n} \cdot \vec{v}_2)^3 + \frac{1}{2} \vec{S}_1 \times \vec{v}_1 \cdot \vec{v}_2 (\hat{n} \cdot \vec{v}_2)^2 - \frac{1}{2} \vec{a}_1 \times \vec{S}_1 \cdot \vec{v}_2 (\hat{n} \cdot \vec{v}_2)^2 + \right. \\ & \frac{5}{3} \hat{n} \times \vec{S}_1 \cdot \vec{v}_1 (\hat{n} \cdot \vec{v}_1)^2 \hat{n} \cdot \vec{v}_2 - 2 \hat{n} \times \vec{a}_1 \cdot \vec{S}_1 (\hat{n} \cdot \vec{v}_1)^2 \hat{n} \cdot \vec{v}_2 + \vec{a}_1 \times \vec{S}_1 \cdot \vec{v}_1 \hat{n} \cdot \vec{v}_1 \hat{n} \cdot \vec{v}_2 - \\ & \frac{1}{3} \vec{a}_2 \times \vec{S}_1 \cdot \vec{v}_1 \hat{n} \cdot \vec{v}_1 \hat{n} \cdot \vec{v}_2 + 2 \hat{n} \times \vec{S}_1 \cdot \vec{v}_1 \hat{n} \cdot \vec{a}_1 \hat{n} \cdot \vec{v}_1 \hat{n} \cdot \vec{v}_2 + \frac{4}{3} \hat{n} \times \vec{S}_1 \cdot \vec{v}_1 \hat{n} \cdot \vec{a}_2 \hat{n} \cdot \vec{v}_1 \hat{n} \cdot \vec{v}_2 - \\ & \hat{n} \times \vec{S}_1 \cdot \vec{v}_1 \vec{a}_1 \cdot \vec{v}_1 \hat{n} \cdot \vec{v}_2 - \frac{1}{3} \hat{n} \times \vec{S}_1 \cdot \vec{v}_1 \vec{a}_2 \cdot \vec{v}_1 \hat{n} \cdot \vec{v}_2 - \frac{2}{3} \hat{n} \times \vec{S}_1 \cdot \vec{v}_1 \vec{v}_1 \cdot \vec{v}_1 \hat{n} \cdot \vec{v}_2 + \frac{3}{4} \hat{n} \times \vec{a}_1 \cdot \vec{S}_1 \vec{v}_1 \cdot \vec{v}_1 \hat{n} \cdot \vec{v}_2 - \\ & \frac{1}{2} \hat{n} \times \vec{S}_1 \cdot \vec{v}_1 \vec{v}_2 \cdot \vec{v}_2 \hat{n} \cdot \vec{v}_2 + \frac{1}{2} \hat{n} \times \vec{a}_1 \cdot \vec{S}_1 \vec{v}_2 \cdot \vec{v}_2 \hat{n} \cdot \vec{v}_2 - \frac{5}{12} \vec{S}_1 \times \vec{v}_1 \cdot \vec{v}_2 (\hat{n} \cdot \vec{v}_1)^2 + \frac{1}{2} \vec{a}_1 \times \vec{S}_1 \cdot \vec{v}_2 (\hat{n} \cdot \vec{v}_1)^2 - \\ & \frac{1}{2} \vec{S}_1 \times \vec{v}_1 \cdot \vec{v}_2 \hat{n} \cdot \vec{a}_1 \hat{n} \cdot \vec{v}_1 - \frac{1}{3} \vec{S}_1 \times \vec{v}_1 \cdot \vec{v}_2 \hat{n} \cdot \vec{a}_2 \hat{n} \cdot \vec{v}_1 + \frac{1}{2} \vec{S}_1 \times \vec{v}_1 \cdot \vec{v}_2 \vec{a}_1 \cdot \vec{v}_1 - \frac{1}{2} \hat{n} \times \vec{S}_1 \cdot \vec{v}_1 \hat{n} \cdot \vec{v}_1 \vec{a}_1 \cdot \vec{v}_2 + \\ & \frac{1}{6} \vec{S}_1 \times \vec{v}_1 \cdot \vec{v}_2 \vec{a}_2 \cdot \vec{v}_1 + \frac{5}{3} \hat{n} \times \vec{S}_1 \cdot \vec{v}_1 \hat{n} \cdot \vec{v}_1 \vec{a}_2 \cdot \vec{v}_2 + \frac{1}{3} \vec{S}_1 \times \vec{v}_1 \cdot \vec{v}_2 \vec{v}_1 \cdot \vec{v}_1 - \frac{3}{8} \vec{a}_1 \times \vec{S}_1 \cdot \vec{v}_2 \vec{v}_1 \cdot \vec{v}_1 - \\ & \frac{1}{2} \vec{a}_1 \times \vec{S}_1 \cdot \vec{v}_1 \vec{v}_1 \cdot \vec{v}_2 + \frac{1}{6} \vec{a}_2 \times \vec{S}_1 \cdot \vec{v}_1 \vec{v}_1 \cdot \vec{v}_2 - \frac{1}{2} \hat{n} \times \vec{S}_1 \cdot \vec{v}_1 \hat{n} \cdot \vec{a}_1 \vec{v}_1 \cdot \vec{v}_2 - \frac{1}{3} \hat{n} \times \vec{S}_1 \cdot \vec{v}_1 \hat{n} \cdot \vec{a}_2 \vec{v}_1 \cdot \vec{v}_2 - \\ & \left. \frac{5}{6} \hat{n} \times \vec{S}_1 \cdot \vec{v}_1 \hat{n} \cdot \vec{v}_1 \vec{v}_1 \cdot \vec{v}_2 + \hat{n} \times \vec{a}_1 \cdot \vec{S}_1 \hat{n} \cdot \vec{v}_1 \vec{v}_1 \cdot \vec{v}_2 + \frac{1}{4} \vec{S}_1 \times \vec{v}_1 \cdot \vec{v}_2 \vec{v}_2 \cdot \vec{v}_2 - \frac{1}{4} \vec{a}_1 \times \vec{S}_1 \cdot \vec{v}_2 \vec{v}_2 \cdot \vec{v}_2 \right) m_2^2 + \\ & \frac{1}{r^3} G^2 \left( \frac{2}{3} \vec{S}_1 \times \vec{v}_1 \cdot \vec{v}_2 (\hat{n} \cdot \vec{v}_1)^3 - 4 \hat{n} \times \vec{S}_1 \cdot \vec{v}_1 \hat{n} \cdot \vec{v}_2 (\hat{n} \cdot \vec{v}_1)^3 + 2 \hat{n} \times \vec{S}_1 \cdot \vec{v}_1 \vec{v}_1 \cdot \vec{v}_2 (\hat{n} \cdot \vec{v}_1)^2 + \right. \\ & 4 \hat{n} \times \vec{S}_1 \cdot \vec{v}_1 (\hat{n} \cdot \vec{v}_2)^3 \hat{n} \cdot \vec{v}_1 - 2 \vec{S}_1 \times \vec{v}_1 \cdot \vec{v}_2 (\hat{n} \cdot \vec{v}_2)^2 \hat{n} \cdot \vec{v}_1 - \frac{3}{4} \vec{S}_1 \times \vec{v}_1 \cdot \vec{v}_2 \vec{v}_1 \cdot \vec{v}_1 \hat{n} \cdot \vec{v}_1 + \\ & 3 \hat{n} \times \vec{S}_1 \cdot \vec{v}_1 \hat{n} \cdot \vec{v}_2 \vec{v}_1 \cdot \vec{v}_1 \hat{n} \cdot \vec{v}_1 - \frac{1}{2} \vec{S}_1 \times \vec{v}_1 \cdot \vec{v}_2 \vec{v}_2 \cdot \vec{v}_2 \hat{n} \cdot \vec{v}_1 + 2 \hat{n} \times \vec{S}_1 \cdot \vec{v}_1 \hat{n} \cdot \vec{v}_2 \vec{v}_2 \cdot \vec{v}_2 \hat{n} \cdot \vec{v}_1 - \\ & \left. 2 \hat{n} \times \vec{S}_1 \cdot \vec{v}_1 (\hat{n} \cdot \vec{v}_2)^2 \vec{v}_1 \cdot \vec{v}_2 + \vec{S}_1 \times \vec{v}_1 \cdot \vec{v}_2 \hat{n} \cdot \vec{v}_2 \vec{v}_1 \cdot \vec{v}_2 - \frac{3}{4} \hat{n} \times \vec{S}_1 \cdot \vec{v}_1 \vec{v}_1 \cdot \vec{v}_1 \vec{v}_1 \cdot \vec{v}_2 - \frac{1}{2} \hat{n} \times \vec{S}_1 \cdot \vec{v}_1 \vec{v}_1 \cdot \vec{v}_2 \vec{v}_2 \cdot \vec{v}_2 \right) m_2^2 \} \end{aligned}$$

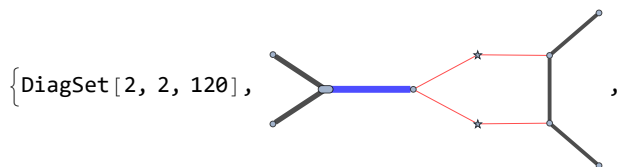

[illegible]

`DiagSet[2, 2, 121],`

Printed by Wolfram Mathematica Student Edition



[illegible]

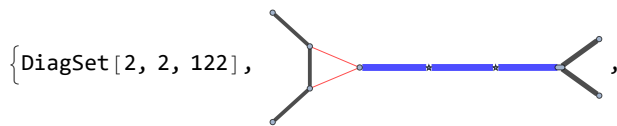

$$\begin{aligned}
 & \frac{1}{r} G^2 \left( \frac{1}{6} \hat{n} \times \vec{a}_1 \cdot \vec{S}_1 (\hat{n} \cdot \vec{v}_2)^2 - \frac{1}{6} \hat{n} \times \vec{S}_1 \cdot \vec{v}_1 (\hat{n} \cdot \vec{v}_2)^2 + \frac{1}{3} \hat{n} \times \vec{a}_1 \cdot \vec{S}_1 (\hat{n} \cdot \vec{v}_2)^2 - \frac{1}{6} \vec{a}_1 \times \vec{S}_1 \cdot \vec{v}_2 \hat{n} \cdot \vec{v}_2 + \frac{1}{6} \vec{S}_1 \times \vec{v}_1 \cdot \vec{v}_2 \hat{n} \cdot \vec{v}_2 - \right. \\
 & \quad \frac{1}{3} \vec{a}_1 \times \vec{S}_1 \cdot \vec{v}_2 \hat{n} \cdot \vec{v}_2 - \frac{1}{12} \vec{a}_2 \times \vec{S}_1 \cdot \vec{v}_1 \hat{n} \cdot \vec{a}_1 + \frac{1}{12} \vec{a}_1 \times \vec{S}_1 \cdot \vec{v}_1 \hat{n} \cdot \vec{a}_2 + \frac{1}{6} \hat{n} \times \vec{S}_1 \cdot \vec{v}_1 \hat{n} \cdot \vec{a}_1 \hat{n} \cdot \vec{a}_2 - \frac{1}{6} \vec{a}_1 \times \vec{a}_2 \cdot \vec{S}_1 \hat{n} \cdot \vec{v}_1 - \\
 & \quad \frac{1}{6} \vec{a}_2 \times \vec{S}_1 \cdot \vec{v}_1 \hat{n} \cdot \vec{v}_1 + \frac{1}{3} \hat{n} \times \vec{S}_1 \cdot \vec{v}_1 \hat{n} \cdot \vec{a}_2 \hat{n} \cdot \vec{v}_1 - \frac{1}{3} \hat{n} \times \vec{a}_1 \cdot \vec{S}_1 \hat{n} \cdot \vec{a}_2 \hat{n} \cdot \vec{v}_1 - \frac{1}{12} \hat{n} \times \vec{S}_1 \cdot \vec{v}_1 \vec{a}_1 \cdot \vec{a}_2 - \\
 & \quad \left. \frac{1}{6} \hat{n} \times \vec{S}_1 \cdot \vec{v}_1 \vec{a}_2 \cdot \vec{v}_1 + \frac{1}{6} \hat{n} \times \vec{a}_1 \cdot \vec{S}_1 \vec{a}_2 \cdot \vec{v}_1 - \frac{1}{12} \hat{n} \times \vec{a}_1 \cdot \vec{S}_1 \vec{v}_2 \cdot \vec{v}_2 + \frac{1}{12} \hat{n} \times \vec{S}_1 \cdot \vec{v}_1 \vec{v}_2 \cdot \vec{v}_2 - \frac{1}{6} \hat{n} \times \vec{a}_1 \cdot \vec{S}_1 \vec{v}_2 \cdot \vec{v}_2 \right) m_2^2 + \\
 & \frac{1}{r^2} G^2 \left( \frac{1}{6} \vec{a}_2 \times \vec{S}_1 \cdot \vec{v}_1 (\hat{n} \cdot \vec{v}_1)^2 - \frac{2}{3} \hat{n} \times \vec{S}_1 \cdot \vec{v}_1 \hat{n} \cdot \vec{a}_2 (\hat{n} \cdot \vec{v}_1)^2 + \frac{4}{3} \hat{n} \times \vec{S}_1 \cdot \vec{v}_1 (\hat{n} \cdot \vec{v}_2)^2 \hat{n} \cdot \vec{v}_1 - \right. \\
 & \quad \frac{4}{3} \hat{n} \times \vec{a}_1 \cdot \vec{S}_1 (\hat{n} \cdot \vec{v}_2)^2 \hat{n} \cdot \vec{v}_1 - \frac{2}{3} \vec{S}_1 \times \vec{v}_1 \cdot \vec{v}_2 \hat{n} \cdot \vec{v}_2 \hat{n} \cdot \vec{v}_1 + \frac{2}{3} \vec{a}_1 \times \vec{S}_1 \cdot \vec{v}_2 \hat{n} \cdot \vec{v}_2 \hat{n} \cdot \vec{v}_1 + \\
 & \quad \frac{1}{3} \hat{n} \times \vec{S}_1 \cdot \vec{v}_1 \vec{a}_2 \cdot \vec{v}_1 \hat{n} \cdot \vec{v}_1 - \frac{1}{3} \hat{n} \times \vec{S}_1 \cdot \vec{v}_1 \vec{v}_2 \cdot \vec{v}_2 \hat{n} \cdot \vec{v}_1 + \frac{1}{3} \hat{n} \times \vec{a}_1 \cdot \vec{S}_1 \vec{v}_2 \cdot \vec{v}_2 \hat{n} \cdot \vec{v}_1 + \frac{1}{6} \vec{a}_1 \times \vec{S}_1 \cdot \vec{v}_1 (\hat{n} \cdot \vec{v}_2)^2 + \\
 & \quad \frac{2}{3} \hat{n} \times \vec{S}_1 \cdot \vec{v}_1 \hat{n} \cdot \vec{a}_1 (\hat{n} \cdot \vec{v}_2)^2 - \frac{1}{3} \vec{S}_1 \times \vec{v}_1 \cdot \vec{v}_2 \hat{n} \cdot \vec{a}_1 \hat{n} \cdot \vec{v}_2 + \frac{1}{6} \vec{S}_1 \times \vec{v}_1 \cdot \vec{v}_2 \vec{a}_1 \cdot \vec{v}_2 - \frac{1}{3} \hat{n} \times \vec{S}_1 \cdot \vec{v}_1 \hat{n} \cdot \vec{v}_2 \vec{a}_1 \cdot \vec{v}_2 - \\
 & \quad \frac{1}{12} \vec{a}_2 \times \vec{S}_1 \cdot \vec{v}_1 \vec{v}_1 \cdot \vec{v}_1 + \frac{1}{6} \hat{n} \times \vec{S}_1 \cdot \vec{v}_1 \hat{n} \cdot \vec{a}_2 \vec{v}_1 \cdot \vec{v}_1 + \frac{1}{3} \vec{S}_1 \times \vec{v}_1 \cdot \vec{v}_2 \vec{v}_1 \cdot \vec{v}_2 - \frac{1}{3} \vec{a}_1 \times \vec{S}_1 \cdot \vec{v}_2 \vec{v}_1 \cdot \vec{v}_2 - \\
 & \quad \left. \frac{2}{3} \hat{n} \times \vec{S}_1 \cdot \vec{v}_1 \hat{n} \cdot \vec{v}_2 \vec{v}_1 \cdot \vec{v}_2 + \frac{2}{3} \hat{n} \times \vec{a}_1 \cdot \vec{S}_1 \hat{n} \cdot \vec{v}_2 \vec{v}_1 \cdot \vec{v}_2 - \frac{1}{12} \vec{a}_1 \times \vec{S}_1 \cdot \vec{v}_1 \vec{v}_2 \cdot \vec{v}_2 - \frac{1}{6} \hat{n} \times \vec{S}_1 \cdot \vec{v}_1 \hat{n} \cdot \vec{a}_1 \vec{v}_2 \cdot \vec{v}_2 \right) m_2^2 + \\
 & \frac{1}{r^3} G^2 \left( -4 \hat{n} \times \vec{S}_1 \cdot \vec{v}_1 (\hat{n} \cdot \vec{v}_2)^2 (\hat{n} \cdot \vec{v}_1)^2 + \frac{4}{3} \vec{S}_1 \times \vec{v}_1 \cdot \vec{v}_2 \hat{n} \cdot \vec{v}_2 (\hat{n} \cdot \vec{v}_1)^2 + \frac{2}{3} \hat{n} \times \vec{S}_1 \cdot \vec{v}_1 \vec{v}_2 \cdot \vec{v}_2 (\hat{n} \cdot \vec{v}_1)^2 - \right. \\
 & \quad \frac{2}{3} \vec{S}_1 \times \vec{v}_1 \cdot \vec{v}_2 \vec{v}_1 \cdot \vec{v}_2 \hat{n} \cdot \vec{v}_1 + \frac{8}{3} \hat{n} \times \vec{S}_1 \cdot \vec{v}_1 \hat{n} \cdot \vec{v}_2 \vec{v}_1 \cdot \vec{v}_2 \hat{n} \cdot \vec{v}_1 - \frac{1}{3} \hat{n} \times \vec{S}_1 \cdot \vec{v}_1 (\vec{v}_1 \cdot \vec{v}_2)^2 + \\
 & \quad \left. \frac{2}{3} \hat{n} \times \vec{S}_1 \cdot \vec{v}_1 (\hat{n} \cdot \vec{v}_2)^2 \vec{v}_1 \cdot \vec{v}_1 - \frac{1}{3} \vec{S}_1 \times \vec{v}_1 \cdot \vec{v}_2 \hat{n} \cdot \vec{v}_2 \vec{v}_1 \cdot \vec{v}_1 - \frac{1}{6} \hat{n} \times \vec{S}_1 \cdot \vec{v}_1 \vec{v}_1 \cdot \vec{v}_1 \vec{v}_2 \cdot \vec{v}_2 \right) m_2^2 + \\
 & G^2 \left( -\frac{1}{12} \log\left(\frac{r}{R_\theta}\right) \vec{a}_1 \times \vec{a}_2 \cdot \vec{S}_1 + \frac{1}{18} \vec{a}_1 \times \vec{a}_2 \cdot \vec{S}_1 + \frac{1}{9} \vec{a}_1 \times \vec{a}_2 \cdot \vec{S}_1 + \frac{1}{18} \vec{a}_2 \times \vec{S}_1 \cdot \vec{v}_1 + \frac{1}{12} \hat{n} \times \vec{a}_1 \cdot \vec{S}_1 \hat{n} \cdot \vec{a}_2 - \right. \\
 & \quad \frac{1}{12} \hat{n} \times \vec{S}_1 \cdot \vec{v}_1 \hat{n} \cdot \vec{a}_2 + \frac{1}{6} \hat{n} \times \vec{a}_1 \cdot \vec{S}_1 \hat{n} \cdot \vec{a}_2 - \frac{1}{6} \vec{a}_1 \times \vec{a}_2 \cdot \vec{S}_1 \log\left(\frac{r}{R_\theta}\right) - \\
 & \quad \left. \frac{1}{12} \vec{a}_2 \times \vec{S}_1 \cdot \vec{v}_1 \log\left(\frac{r}{R_\theta}\right) + \frac{\frac{1}{24} \vec{a}_1 \times \vec{a}_2 \cdot \vec{S}_1 + \frac{1}{12} \vec{a}_1 \times \vec{a}_2 \cdot \vec{S}_1 + \frac{1}{24} \vec{a}_2 \times \vec{S}_1 \cdot \vec{v}_1}{\epsilon_d} \right) m_2^2 \Big\}
 \end{aligned}$$

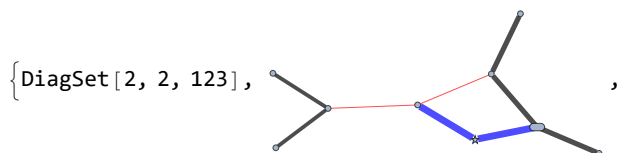

$$\begin{aligned}
 & \frac{1}{r} \left( 7 \hat{n} \times \vec{S}_1 \cdot \vec{a}_1 (\hat{n} \cdot \vec{v}_1)^2 + 3 \hat{n} \times \vec{S}_1 \cdot \vec{v}_1 (\hat{n} \cdot \vec{v}_1)^2 + 4 \hat{n} \times \vec{S}_1 \cdot \vec{a}_1 (\hat{n} \cdot \vec{v}_1)^2 + \frac{7}{3} \vec{S}_1 \times \vec{a}_1 \cdot \vec{v}_2 \hat{n} \cdot \vec{v}_1 + \frac{11}{4} \vec{S}_1 \times \vec{v}_1 \cdot \vec{a}_1 \hat{n} \cdot \vec{v}_1 - \right. \\
 & \quad \frac{1}{3} \vec{S}_1 \times \vec{v}_1 \cdot \vec{a}_2 \hat{n} \cdot \vec{v}_1 + \frac{2}{3} \vec{S}_1 \times \vec{v}_1 \cdot \vec{v}_2 \hat{n} \cdot \vec{v}_1 + \frac{4}{3} \vec{S}_1 \times \vec{a}_1 \cdot \vec{v}_2 \hat{n} \cdot \vec{v}_1 - \frac{1}{3} \vec{S}_1 \times \vec{a}_1 \cdot \vec{a}_2 \hat{n} \cdot \vec{v}_1 + 2 \vec{S}_1 \times \vec{v}_1 \cdot \vec{a}_1 \hat{n} \cdot \vec{v}_1 + \\
 & \quad \left. 2 \hat{n} \times \vec{S}_1 \cdot \vec{v}_1 \hat{n} \cdot \vec{a}_1 \hat{n} \cdot \vec{v}_1 + 5 \hat{n} \times \vec{S}_1 \cdot \vec{v}_1 \hat{n} \cdot \vec{a}_1 \hat{n} \cdot \vec{v}_1 + 6 \hat{n} \times \vec{S}_1 \cdot \vec{a}_1 \hat{n} \cdot \vec{a}_1 \hat{n} \cdot \vec{v}_1 + \frac{2}{3} \hat{n} \times \vec{S}_1 \cdot \vec{v}_1 \hat{n} \cdot \vec{a}_2 \hat{n} \cdot \vec{v}_1 + \right.
 \end{aligned}$$

[illegible]

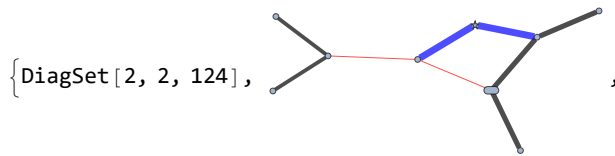

$$\begin{aligned} & \frac{1}{r^2} G^2 m_1 m_2 \left( 4 (\hat{n} \cdot \vec{v}_1)^3 \hat{n} \times \vec{S}_1 \cdot \vec{a}_1 + 8 (\hat{n} \cdot \vec{v}_1)^2 \vec{S}_1 \times \vec{v}_1 \cdot \vec{a}_1 - 40 \hat{n} \cdot \vec{a}_1 (\hat{n} \cdot \vec{v}_1)^2 \hat{n} \times \vec{S}_1 \cdot \vec{v}_1 - 8 \hat{n} \cdot \vec{a}_1 \hat{n} \cdot \vec{v}_1 \vec{S}_1 \times \vec{v}_1 \cdot \vec{v}_2 - \right. \\ & 4 \hat{n} \cdot \vec{v}_2 \hat{n} \cdot \vec{v}_1 \vec{S}_1 \times \vec{v}_1 \cdot \vec{a}_1 + 32 \hat{n} \cdot \vec{a}_1 \hat{n} \cdot \vec{v}_2 \hat{n} \cdot \vec{v}_1 \hat{n} \times \vec{S}_1 \cdot \vec{v}_1 - 8 \vec{a}_1 \cdot \vec{v}_2 \hat{n} \cdot \vec{v}_1 \hat{n} \times \vec{S}_1 \cdot \vec{v}_1 + \\ & 17 \vec{v}_1 \cdot \vec{a}_1 \hat{n} \cdot \vec{v}_1 \hat{n} \times \vec{S}_1 \cdot \vec{v}_1 - 8 \vec{v}_1 \cdot \vec{a}_1 \hat{n} \cdot \vec{v}_2 \hat{n} \times \vec{S}_1 \cdot \vec{v}_1 + 7 \vec{v}_1 \cdot \vec{v}_1 \hat{n} \cdot \vec{a}_1 \hat{n} \times \vec{S}_1 \cdot \vec{v}_1 - 8 \vec{v}_1 \cdot \vec{v}_2 \hat{n} \cdot \vec{a}_1 \hat{n} \times \vec{S}_1 \cdot \vec{v}_1 + \\ & \left. 4 \vec{v}_1 \cdot \vec{a}_1 \vec{S}_1 \times \vec{v}_1 \cdot \vec{v}_2 - \vec{v}_1 \cdot \vec{v}_1 \vec{S}_1 \times \vec{v}_1 \cdot \vec{a}_1 + 2 \vec{v}_1 \cdot \vec{v}_2 \vec{S}_1 \times \vec{v}_1 \cdot \vec{a}_1 + 4 (\hat{n} \cdot \vec{v}_1)^3 \hat{n} \times \vec{S}_1 \cdot \vec{v}_1 \right) + \\ & \frac{1}{r} G^2 m_1 m_2 \left( 2 \hat{n} \cdot \vec{a}_1 \vec{S}_1 \times \vec{v}_1 \cdot \vec{a}_1 + 8 \hat{n} \cdot \vec{a}_1 \hat{n} \cdot \vec{v}_1 \hat{n} \times \vec{S}_1 \cdot \vec{v}_1 + 8 \hat{n} \cdot \vec{a}_1 \hat{n} \cdot \vec{v}_1 \hat{n} \times \vec{S}_1 \cdot \vec{a}_1 - \right. \\ & \left. 2 \hat{n} \cdot \vec{v}_1 \vec{S}_1 \times \vec{v}_1 \cdot \vec{a}_1 - 4 \vec{v}_1 \cdot \vec{a}_1 \hat{n} \times \vec{S}_1 \cdot \vec{v}_1 - 4 \vec{v}_1 \cdot \vec{a}_1 \hat{n} \times \vec{S}_1 \cdot \vec{a}_1 \right) + \frac{1}{r^3} \\ & G^2 m_1 m_2 \left( -20 (\hat{n} \cdot \vec{v}_1)^4 \hat{n} \times \vec{S}_1 \cdot \vec{v}_1 - 4 (\hat{n} \cdot \vec{v}_1)^3 \vec{S}_1 \times \vec{v}_1 \cdot \vec{v}_2 + 24 \hat{n} \cdot \vec{v}_2 (\hat{n} \cdot \vec{v}_1)^3 \hat{n} \times \vec{S}_1 \cdot \vec{v}_1 + \right. \\ & \left. 2 \vec{v}_1 \cdot \vec{v}_1 (\hat{n} \cdot \vec{v}_1)^2 \hat{n} \times \vec{S}_1 \cdot \vec{v}_1 - 12 \vec{v}_1 \cdot \vec{v}_2 (\hat{n} \cdot \vec{v}_1)^2 \hat{n} \times \vec{S}_1 \cdot \vec{v}_1 + 2 (\vec{v}_1 \cdot \vec{v}_1)^2 \hat{n} \times \vec{S}_1 \cdot \vec{v}_1 \right) \} \end{aligned}$$

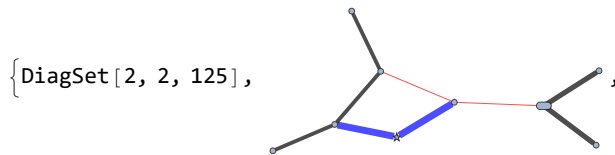

$$\begin{aligned} & \frac{1}{r} G^2 \left( -\frac{8}{3} \vec{S}_1 \times \vec{v}_1 \cdot \vec{v}_2 \hat{n} \cdot \vec{a}_2 + \frac{8}{3} \vec{a}_1 \times \vec{S}_1 \cdot \vec{v}_2 \hat{n} \cdot \vec{a}_2 + \frac{16}{3} \hat{n} \times \vec{S}_1 \cdot \vec{v}_1 \hat{n} \cdot \vec{v}_2 \hat{n} \cdot \vec{a}_2 - \frac{16}{3} \hat{n} \times \vec{a}_1 \cdot \vec{S}_1 \hat{n} \cdot \vec{v}_2 \hat{n} \cdot \vec{a}_2 - \right. \\ & \left. \frac{8}{3} \vec{a}_1 \times \vec{a}_2 \cdot \vec{S}_1 \hat{n} \cdot \vec{v}_2 - \frac{8}{3} \vec{a}_2 \times \vec{S}_1 \cdot \vec{v}_1 \hat{n} \cdot \vec{v}_2 - \frac{8}{3} \hat{n} \times \vec{S}_1 \cdot \vec{v}_1 \vec{a}_2 \cdot \vec{v}_2 + \frac{8}{3} \hat{n} \times \vec{a}_1 \cdot \vec{S}_1 \vec{a}_2 \cdot \vec{v}_2 \right) m_2^2 + \frac{1}{r^2} \\ & G^2 \left( -\frac{16}{3} \hat{n} \times \vec{S}_1 \cdot \vec{v}_1 (\hat{n} \cdot \vec{v}_2)^3 + \frac{16}{3} \hat{n} \times \vec{a}_1 \cdot \vec{S}_1 (\hat{n} \cdot \vec{v}_2)^3 + 4 \vec{S}_1 \times \vec{v}_1 \cdot \vec{v}_2 (\hat{n} \cdot \vec{v}_2)^2 - 4 \vec{a}_1 \times \vec{S}_1 \cdot \vec{v}_2 (\hat{n} \cdot \vec{v}_2)^2 - \right. \\ & 8 \vec{a}_2 \times \vec{S}_1 \cdot \vec{v}_1 (\hat{n} \cdot \vec{v}_2)^2 + 32 \hat{n} \times \vec{S}_1 \cdot \vec{v}_1 \hat{n} \cdot \vec{a}_2 (\hat{n} \cdot \vec{v}_2)^2 - 16 \vec{S}_1 \times \vec{v}_1 \cdot \vec{v}_2 \hat{n} \cdot \vec{a}_2 \hat{n} \cdot \vec{v}_2 + \frac{16}{3} \vec{a}_2 \times \vec{S}_1 \cdot \vec{v}_1 \hat{n} \cdot \vec{v}_1 \hat{n} \cdot \vec{v}_2 - \\ & \frac{64}{3} \hat{n} \times \vec{S}_1 \cdot \vec{v}_1 \hat{n} \cdot \vec{a}_2 \hat{n} \cdot \vec{v}_1 \hat{n} \cdot \vec{v}_2 + \frac{16}{3} \hat{n} \times \vec{S}_1 \cdot \vec{v}_1 \vec{a}_2 \cdot \vec{v}_1 \hat{n} \cdot \vec{v}_2 - 12 \hat{n} \times \vec{S}_1 \cdot \vec{v}_1 \vec{a}_2 \cdot \vec{v}_2 \hat{n} \cdot \vec{v}_2 + \\ & \frac{16}{3} \vec{S}_1 \times \vec{v}_1 \cdot \vec{v}_2 \hat{n} \cdot \vec{a}_2 \hat{n} \cdot \vec{v}_1 - \frac{8}{3} \vec{S}_1 \times \vec{v}_1 \cdot \vec{v}_2 \vec{a}_2 \cdot \vec{v}_1 + 6 \vec{S}_1 \times \vec{v}_1 \cdot \vec{v}_2 \vec{a}_2 \cdot \vec{v}_2 + \frac{16}{3} \hat{n} \times \vec{S}_1 \cdot \vec{v}_1 \hat{n} \cdot \vec{v}_1 \vec{a}_2 \cdot \vec{v}_2 - \\ & \left. \frac{8}{3} \vec{a}_2 \times \vec{S}_1 \cdot \vec{v}_1 \vec{v}_1 \cdot \vec{v}_2 + \frac{16}{3} \hat{n} \times \vec{S}_1 \cdot \vec{v}_1 \hat{n} \cdot \vec{a}_2 \vec{v}_1 \cdot \vec{v}_2 + 2 \vec{a}_2 \times \vec{S}_1 \cdot \vec{v}_1 \vec{v}_2 \cdot \vec{v}_2 - 4 \hat{n} \times \vec{S}_1 \cdot \vec{v}_1 \hat{n} \cdot \vec{a}_2 \vec{v}_2 \cdot \vec{v}_2 \right) m_2^2 + \\ & \frac{1}{r^3} G^2 \left( -24 \hat{n} \times \vec{S}_1 \cdot \vec{v}_1 (\hat{n} \cdot \vec{v}_2)^4 + 16 \vec{S}_1 \times \vec{v}_1 \cdot \vec{v}_2 (\hat{n} \cdot \vec{v}_2)^3 + 32 \hat{n} \times \vec{S}_1 \cdot \vec{v}_1 \hat{n} \cdot \vec{v}_1 (\hat{n} \cdot \vec{v}_2)^3 - \right. \\ & 16 \vec{S}_1 \times \vec{v}_1 \cdot \vec{v}_2 \hat{n} \cdot \vec{v}_1 (\hat{n} \cdot \vec{v}_2)^2 - 16 \hat{n} \times \vec{S}_1 \cdot \vec{v}_1 \vec{v}_1 \cdot \vec{v}_2 (\hat{n} \cdot \vec{v}_2)^2 + 4 \hat{n} \times \vec{S}_1 \cdot \vec{v}_1 \vec{v}_2 \cdot \vec{v}_2 (\hat{n} \cdot \vec{v}_2)^2 + \\ & \left. 8 \vec{S}_1 \times \vec{v}_1 \cdot \vec{v}_2 \vec{v}_1 \cdot \vec{v}_2 \hat{n} \cdot \vec{v}_2 - 2 \vec{S}_1 \times \vec{v}_1 \cdot \vec{v}_2 \vec{v}_2 \cdot \vec{v}_2 \hat{n} \cdot \vec{v}_2 + 2 \hat{n} \times \vec{S}_1 \cdot \vec{v}_1 (\vec{v}_2 \cdot \vec{v}_2)^2 \right) m_2^2 \} \end{aligned}$$

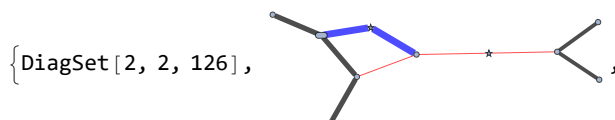

$$\begin{aligned} & \frac{1}{r} \left( \frac{2}{3} \hat{n} \times \vec{S}_1 \cdot \vec{a}_1 (\hat{n} \cdot \vec{v}_2)^2 + \frac{1}{3} \hat{n} \times \vec{S}_1 \cdot \vec{v}_1 (\hat{n} \cdot \vec{v}_2)^2 + \frac{1}{3} \hat{n} \times \vec{S}_1 \cdot \vec{a}_1 (\hat{n} \cdot \vec{v}_2)^2 - \frac{2}{3} \vec{S}_1 \times \vec{a}_1 \cdot \vec{v}_2 \hat{n} \cdot \vec{v}_2 + \frac{1}{6} \vec{S}_1 \times \vec{v}_1 \cdot \vec{a}_1 \hat{n} \cdot \vec{v}_2 - \right. \\ & \left. \frac{1}{3} \vec{S}_1 \times \vec{v}_1 \cdot \vec{v}_2 \hat{n} \cdot \vec{v}_2 - \frac{1}{3} \vec{S}_1 \times \vec{a}_1 \cdot \vec{v}_2 \hat{n} \cdot \vec{v}_2 + \frac{1}{6} \vec{S}_1 \times \vec{v}_1 \cdot \vec{a}_1 \hat{n} \cdot \vec{v}_2 - \frac{7}{12} \hat{n} \times \vec{S}_1 \cdot \vec{v}_1 \hat{n} \cdot \vec{a}_1 \hat{n} \cdot \vec{v}_2 - \right. \end{aligned}$$

[illegible]

$$\frac{1}{6} \vec{S}_1 \times \vec{a}_1 \cdot \vec{a}_2 \log \left( \frac{r}{R_0} \right) + \frac{-\frac{1}{6} \vec{S}_1 \times \vec{a}_1 \cdot \vec{a}_2 - \frac{1}{12} \vec{S}_1 \times \vec{v}_1 \cdot \vec{a}_2 - \frac{1}{12} \vec{S}_1 \times \vec{a}_1 \cdot \vec{a}_2}{\epsilon_d} \Bigg\} G^2 \Bigg\}$$

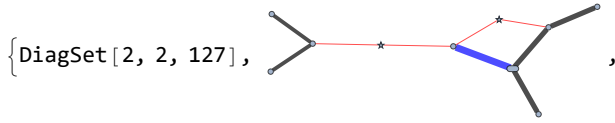

$$\begin{aligned} & \frac{1}{r} \left( \frac{5}{24} \vec{S}_1 \times \vec{v}_1 \cdot \vec{v}_2 \hat{n} \cdot \vec{a}_1 - \frac{5}{12} \hat{n} \times \vec{S}_1 \cdot \vec{v}_1 \hat{n} \cdot \vec{v}_2 \hat{n} \cdot \vec{a}_1 + \frac{11}{24} \vec{S}_1 \times \vec{v}_1 \cdot \vec{v}_2 \hat{n} \cdot \vec{a}_1 + \frac{1}{4} \vec{S}_1 \times \vec{a}_1 \cdot \vec{v}_2 \hat{n} \cdot \vec{a}_1 + \frac{1}{4} \vec{S}_1 \times \vec{v}_1 \cdot \vec{a}_2 \hat{n} \cdot \vec{a}_1 - \right. \\ & \quad \frac{1}{2} \hat{n} \times \vec{S}_1 \cdot \vec{v}_1 \hat{n} \cdot \vec{a}_1 \hat{n} \cdot \vec{a}_2 + \frac{7}{24} \vec{S}_1 \times \vec{a}_1 \cdot \vec{v}_2 \hat{n} \cdot \vec{v}_1 + \frac{1}{4} \vec{S}_1 \times \vec{v}_1 \cdot \vec{a}_2 \hat{n} \cdot \vec{v}_1 + \frac{1}{4} \vec{S}_1 \times \vec{v}_1 \cdot \vec{v}_2 \hat{n} \cdot \vec{v}_1 + \frac{1}{24} \vec{S}_1 \times \vec{a}_1 \cdot \vec{v}_2 \hat{n} \cdot \vec{v}_1 + \\ & \quad \frac{1}{4} \vec{S}_1 \times \vec{a}_1 \cdot \vec{a}_2 \hat{n} \cdot \vec{v}_1 - \frac{1}{2} \hat{n} \times \vec{S}_1 \cdot \vec{v}_1 \hat{n} \cdot \vec{a}_2 \hat{n} \cdot \vec{v}_1 - \frac{1}{2} \hat{n} \times \vec{S}_1 \cdot \vec{a}_1 \hat{n} \cdot \vec{a}_2 \hat{n} \cdot \vec{v}_1 + \frac{1}{6} \vec{S}_1 \times \vec{v}_1 \cdot \vec{a}_1 \hat{n} \cdot \vec{v}_2 + \frac{1}{6} \vec{S}_1 \times \vec{v}_1 \cdot \vec{a}_1 \hat{n} \cdot \vec{v}_2 - \\ & \quad \frac{11}{12} \hat{n} \times \vec{S}_1 \cdot \vec{v}_1 \hat{n} \cdot \vec{a}_1 \hat{n} \cdot \vec{v}_2 - \frac{1}{2} \hat{n} \times \vec{S}_1 \cdot \vec{a}_1 \hat{n} \cdot \vec{a}_1 \hat{n} \cdot \vec{v}_2 - \frac{7}{12} \hat{n} \times \vec{S}_1 \cdot \vec{a}_1 \hat{n} \cdot \vec{v}_1 \hat{n} \cdot \vec{v}_2 - \frac{1}{2} \hat{n} \times \vec{S}_1 \cdot \vec{v}_1 \hat{n} \cdot \vec{v}_1 \hat{n} \cdot \vec{v}_2 - \\ & \quad \frac{1}{12} \hat{n} \times \vec{S}_1 \cdot \vec{a}_1 \hat{n} \cdot \vec{v}_1 \hat{n} \cdot \vec{v}_2 + \frac{5}{24} \hat{n} \times \vec{S}_1 \cdot \vec{v}_1 \vec{a}_1 \cdot \vec{v}_2 + \frac{1}{4} \hat{n} \times \vec{S}_1 \cdot \vec{v}_1 \vec{a}_1 \cdot \vec{a}_2 + \frac{11}{24} \hat{n} \times \vec{S}_1 \cdot \vec{v}_1 \vec{a}_1 \cdot \vec{v}_2 + \frac{1}{4} \hat{n} \times \vec{S}_1 \cdot \vec{a}_1 \vec{a}_1 \cdot \vec{v}_2 + \\ & \quad \left. \frac{1}{4} \hat{n} \times \vec{S}_1 \cdot \vec{v}_1 \vec{v}_1 \cdot \vec{a}_2 + \frac{1}{4} \hat{n} \times \vec{S}_1 \cdot \vec{a}_1 \vec{v}_1 \cdot \vec{a}_2 + \frac{7}{24} \hat{n} \times \vec{S}_1 \cdot \vec{a}_1 \vec{v}_1 \cdot \vec{v}_2 + \frac{1}{4} \hat{n} \times \vec{S}_1 \cdot \vec{v}_1 \vec{v}_1 \cdot \vec{v}_2 + \frac{1}{24} \hat{n} \times \vec{S}_1 \cdot \vec{a}_1 \vec{v}_1 \cdot \vec{v}_2 \right) \\ & m_1 m_2 G^2 + \frac{1}{r^2} \left( -\frac{17}{24} \vec{S}_1 \times \vec{v}_1 \cdot \vec{v}_2 (\hat{n} \cdot \vec{v}_1)^2 - \frac{7}{24} \vec{S}_1 \times \vec{a}_1 \cdot \vec{v}_2 (\hat{n} \cdot \vec{v}_1)^2 - \frac{1}{2} \vec{S}_1 \times \vec{v}_1 \cdot \vec{a}_2 (\hat{n} \cdot \vec{v}_1)^2 + \right. \\ & \quad 2 \hat{n} \times \vec{S}_1 \cdot \vec{v}_1 \hat{n} \cdot \vec{a}_2 (\hat{n} \cdot \vec{v}_1)^2 + \frac{17}{6} \hat{n} \times \vec{S}_1 \cdot \vec{v}_1 \hat{n} \cdot \vec{v}_2 (\hat{n} \cdot \vec{v}_1)^2 + \frac{7}{6} \hat{n} \times \vec{S}_1 \cdot \vec{a}_1 \hat{n} \cdot \vec{v}_2 (\hat{n} \cdot \vec{v}_1)^2 - \\ & \quad 2 \hat{n} \times \vec{S}_1 \cdot \vec{v}_1 (\hat{n} \cdot \vec{v}_2)^2 \hat{n} \cdot \vec{v}_1 - 2 \hat{n} \times \vec{S}_1 \cdot \vec{a}_1 (\hat{n} \cdot \vec{v}_2)^2 \hat{n} \cdot \vec{v}_1 - \frac{5}{6} \vec{S}_1 \times \vec{v}_1 \cdot \vec{v}_2 \hat{n} \cdot \vec{a}_1 \hat{n} \cdot \vec{v}_1 + \frac{1}{6} \vec{S}_1 \times \vec{v}_1 \cdot \vec{v}_2 \hat{n} \cdot \vec{v}_2 \hat{n} \cdot \vec{v}_1 + \\ & \quad \vec{S}_1 \times \vec{a}_1 \cdot \vec{v}_2 \hat{n} \cdot \vec{v}_2 \hat{n} \cdot \vec{v}_1 - \frac{1}{4} \vec{S}_1 \times \vec{v}_1 \cdot \vec{a}_1 \hat{n} \cdot \vec{v}_2 \hat{n} \cdot \vec{v}_1 + \frac{10}{3} \hat{n} \times \vec{S}_1 \cdot \vec{v}_1 \hat{n} \cdot \vec{a}_1 \hat{n} \cdot \vec{v}_2 \hat{n} \cdot \vec{v}_1 - \frac{5}{6} \hat{n} \times \vec{S}_1 \cdot \vec{v}_1 \vec{a}_1 \cdot \vec{v}_2 \hat{n} \cdot \vec{v}_1 - \\ & \quad \hat{n} \times \vec{S}_1 \cdot \vec{v}_1 \vec{v}_1 \cdot \vec{a}_2 \hat{n} \cdot \vec{v}_1 - \frac{17}{12} \hat{n} \times \vec{S}_1 \cdot \vec{v}_1 \vec{v}_1 \cdot \vec{v}_2 \hat{n} \cdot \vec{v}_1 - \frac{7}{12} \hat{n} \times \vec{S}_1 \cdot \vec{a}_1 \vec{v}_1 \cdot \vec{v}_2 \hat{n} \cdot \vec{v}_1 + \frac{1}{2} \hat{n} \times \vec{S}_1 \cdot \vec{v}_1 \vec{v}_2 \cdot \vec{v}_2 \hat{n} \cdot \vec{v}_1 + \\ & \quad \frac{1}{2} \hat{n} \times \vec{S}_1 \cdot \vec{a}_1 \vec{v}_2 \cdot \vec{v}_2 \hat{n} \cdot \vec{v}_1 - 2 \hat{n} \times \vec{S}_1 \cdot \vec{v}_1 \hat{n} \cdot \vec{a}_1 (\hat{n} \cdot \vec{v}_2)^2 + \vec{S}_1 \times \vec{v}_1 \cdot \vec{v}_2 \hat{n} \cdot \vec{a}_1 \hat{n} \cdot \vec{v}_2 - \frac{1}{2} \vec{S}_1 \times \vec{v}_1 \cdot \vec{v}_2 \vec{a}_1 \cdot \vec{v}_2 + \\ & \quad \hat{n} \times \vec{S}_1 \cdot \vec{v}_1 \hat{n} \cdot \vec{v}_2 \vec{a}_1 \cdot \vec{v}_2 + \frac{19}{24} \vec{S}_1 \times \vec{v}_1 \cdot \vec{v}_2 \vec{v}_1 \cdot \vec{a}_1 - \frac{19}{12} \hat{n} \times \vec{S}_1 \cdot \vec{v}_1 \hat{n} \cdot \vec{v}_2 \vec{v}_1 \cdot \vec{a}_1 + \frac{13}{24} \vec{S}_1 \times \vec{v}_1 \cdot \vec{v}_2 \vec{v}_1 \cdot \vec{v}_1 + \\ & \quad \frac{1}{3} \vec{S}_1 \times \vec{a}_1 \cdot \vec{v}_2 \vec{v}_1 \cdot \vec{v}_1 + \frac{1}{4} \vec{S}_1 \times \vec{v}_1 \cdot \vec{a}_2 \vec{v}_1 \cdot \vec{v}_1 - \frac{1}{2} \hat{n} \times \vec{S}_1 \cdot \vec{v}_1 \hat{n} \cdot \vec{a}_2 \vec{v}_1 \cdot \vec{v}_1 - \frac{13}{12} \hat{n} \times \vec{S}_1 \cdot \vec{v}_1 \hat{n} \cdot \vec{v}_2 \vec{v}_1 \cdot \vec{v}_1 - \\ & \quad \frac{2}{3} \hat{n} \times \vec{S}_1 \cdot \vec{a}_1 \hat{n} \cdot \vec{v}_2 \vec{v}_1 \cdot \vec{v}_1 - \frac{1}{2} \vec{S}_1 \times \vec{v}_1 \cdot \vec{v}_2 \vec{v}_1 \cdot \vec{v}_2 - \frac{1}{2} \vec{S}_1 \times \vec{a}_1 \cdot \vec{v}_2 \vec{v}_1 \cdot \vec{v}_2 + \frac{1}{8} \vec{S}_1 \times \vec{v}_1 \cdot \vec{a}_1 \vec{v}_1 \cdot \vec{v}_2 - \\ & \quad \frac{5}{6} \hat{n} \times \vec{S}_1 \cdot \vec{v}_1 \hat{n} \cdot \vec{a}_1 \vec{v}_1 \cdot \vec{v}_2 + \hat{n} \times \vec{S}_1 \cdot \vec{v}_1 \hat{n} \cdot \vec{v}_2 \vec{v}_1 \cdot \vec{v}_2 + \hat{n} \times \vec{S}_1 \cdot \vec{a}_1 \hat{n} \cdot \vec{v}_2 \vec{v}_1 \cdot \vec{v}_2 + \frac{1}{2} \hat{n} \times \vec{S}_1 \cdot \vec{v}_1 \hat{n} \cdot \vec{a}_1 \vec{v}_2 \cdot \vec{v}_2 \Bigg) m_1 m_2 G^2 + \\ & \frac{1}{r^3} \left( \frac{5}{6} \vec{S}_1 \times \vec{v}_1 \cdot \vec{v}_2 (\hat{n} \cdot \vec{v}_1)^3 - 5 \hat{n} \times \vec{S}_1 \cdot \vec{v}_1 \hat{n} \cdot \vec{v}_2 (\hat{n} \cdot \vec{v}_1)^3 + 12 \hat{n} \times \vec{S}_1 \cdot \vec{v}_1 (\hat{n} \cdot \vec{v}_2)^2 (\hat{n} \cdot \vec{v}_1)^2 - \right. \\ & \quad 4 \vec{S}_1 \times \vec{v}_1 \cdot \vec{v}_2 \hat{n} \cdot \vec{v}_2 (\hat{n} \cdot \vec{v}_1)^2 + \frac{5}{2} \hat{n} \times \vec{S}_1 \cdot \vec{v}_1 \vec{v}_1 \cdot \vec{v}_2 (\hat{n} \cdot \vec{v}_1)^2 - 2 \hat{n} \times \vec{S}_1 \cdot \vec{v}_1 \vec{v}_2 \cdot \vec{v}_2 (\hat{n} \cdot \vec{v}_1)^2 - \\ & \quad \vec{S}_1 \times \vec{v}_1 \cdot \vec{v}_2 \vec{v}_1 \cdot \vec{v}_1 \hat{n} \cdot \vec{v}_1 + 4 \hat{n} \times \vec{S}_1 \cdot \vec{v}_1 \hat{n} \cdot \vec{v}_2 \vec{v}_1 \cdot \vec{v}_1 \hat{n} \cdot \vec{v}_1 + 2 \vec{S}_1 \times \vec{v}_1 \cdot \vec{v}_2 \vec{v}_1 \cdot \vec{v}_2 \hat{n} \cdot \vec{v}_1 - \\ & \quad 8 \hat{n} \times \vec{S}_1 \cdot \vec{v}_1 \hat{n} \cdot \vec{v}_2 \vec{v}_1 \cdot \vec{v}_2 \hat{n} \cdot \vec{v}_1 + \hat{n} \times \vec{S}_1 \cdot \vec{v}_1 (\vec{v}_1 \cdot \vec{v}_2)^2 - 2 \hat{n} \times \vec{S}_1 \cdot \vec{v}_1 (\hat{n} \cdot \vec{v}_2)^2 \vec{v}_1 \cdot \vec{v}_1 + \\ & \quad \left. \vec{S}_1 \times \vec{v}_1 \cdot \vec{v}_2 \hat{n} \cdot \vec{v}_2 \vec{v}_1 \cdot \vec{v}_1 - \hat{n} \times \vec{S}_1 \cdot \vec{v}_1 \vec{v}_1 \cdot \vec{v}_1 \vec{v}_1 \cdot \vec{v}_2 + \frac{1}{2} \hat{n} \times \vec{S}_1 \cdot \vec{v}_1 \vec{v}_1 \cdot \vec{v}_1 \vec{v}_2 \cdot \vec{v}_2 \right) m_1 m_2 G^2 \Bigg\} \end{aligned}$$

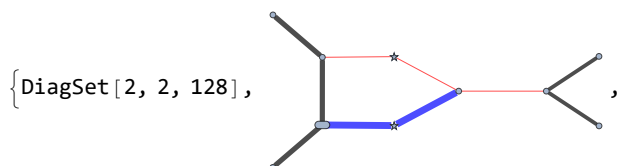

[illegible]

$$\left. \frac{1}{4} \hat{n} \times \vec{S_1} \cdot \vec{a_1} \hat{n} \cdot \vec{v_1} - \frac{1}{6} \vec{S_1} \times \vec{a_1} \cdot \vec{a_1} \log \left( \frac{r}{R_\theta} \right) + \frac{\frac{1}{12} \vec{S_1} \times \vec{a_1} \cdot \vec{a_1} - \frac{1}{12} \vec{S_1} \times \vec{v_1} \cdot \vec{a_1}}{\epsilon_d} \right\} G^2 \}$$

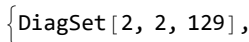

$$\frac{1}{4} \hat{n} \times \vec{S}_1 \cdot \frac{1}{\vec{a}_1} \vec{v}_1 \cdot \vec{v}_2 + \frac{1}{6} \hat{n} \times \vec{S}_1 \cdot \frac{1}{\vec{a}_1} \vec{v}_2 \cdot \vec{v}_2 + \frac{1}{12} \hat{n} \times \vec{S}_1^2 \cdot \vec{v}_1 \vec{v}_2 \cdot \vec{v}_2 + \frac{1}{12} \hat{n} \times \vec{S}_1 \cdot \frac{1}{\vec{a}_1} \vec{v}_2 \cdot \vec{v}_2 \Big) m_1 m_2 G^2 + \frac{1}{r^2}$$



$$\begin{aligned}
& \left( -\frac{23}{3} \hat{n} \times \vec{S}_1 \cdot \vec{v}_1 (\hat{n} \cdot \vec{v}_1)^3 - \frac{13}{4} \hat{n} \times \vec{S}_1 \cdot \vec{a}_1 (\hat{n} \cdot \vec{v}_1)^3 - \frac{37}{12} \vec{S}_1 \times \vec{v}_1 \cdot \vec{v}_2 (\hat{n} \cdot \vec{v}_1)^2 - \frac{11}{8} \vec{S}_1 \times \vec{a}_1 \cdot \vec{v}_2 (\hat{n} \cdot \vec{v}_1)^2 - \right. \\
& \quad \frac{9}{16} \vec{S}_1 \times \vec{v}_1 \cdot \vec{a}_1 (\hat{n} \cdot \vec{v}_1)^2 + \frac{13}{48} \vec{S}_1 \times \vec{v}_1 \cdot \vec{a}_2 (\hat{n} \cdot \vec{v}_1)^2 - \frac{15}{2} \hat{n} \times \vec{S}_1 \cdot \vec{v}_1 \hat{n} \cdot \vec{a}_1 (\hat{n} \cdot \vec{v}_1)^2 - \frac{13}{12} \hat{n} \times \vec{S}_1 \cdot \vec{v}_1 \hat{n} \cdot \vec{a}_2 (\hat{n} \cdot \vec{v}_1)^2 + \\
& \quad \frac{37}{3} \hat{n} \times \vec{S}_1 \cdot \vec{v}_1 \hat{n} \cdot \vec{v}_2 (\hat{n} \cdot \vec{v}_1)^2 + \frac{11}{2} \hat{n} \times \vec{S}_1 \cdot \vec{a}_1 \hat{n} \cdot \vec{v}_2 (\hat{n} \cdot \vec{v}_1)^2 - 4 \hat{n} \times \vec{S}_1 \cdot \vec{v}_1 (\hat{n} \cdot \vec{v}_2)^2 \hat{n} \cdot \vec{v}_1 - \\
& \quad \frac{7}{3} \hat{n} \times \vec{S}_1 \cdot \vec{a}_1 (\hat{n} \cdot \vec{v}_2)^2 \hat{n} \cdot \vec{v}_1 - \frac{13}{4} \vec{S}_1 \times \vec{v}_1 \cdot \vec{v}_2 \hat{n} \cdot \vec{a}_1 \hat{n} \cdot \vec{v}_1 + 2 \vec{S}_1 \times \vec{v}_1 \cdot \vec{v}_2 \hat{n} \cdot \vec{v}_2 \hat{n} \cdot \vec{v}_1 + \frac{7}{6} \vec{S}_1 \times \vec{a}_1 \cdot \vec{v}_2 \hat{n} \cdot \vec{v}_2 \hat{n} \cdot \vec{v}_1 - \\
& \quad \frac{1}{2} \vec{S}_1 \times \vec{v}_1 \cdot \vec{a}_1 \hat{n} \cdot \vec{v}_2 \hat{n} \cdot \vec{v}_1 + 13 \hat{n} \times \vec{S}_1 \cdot \vec{v}_1 \hat{n} \cdot \vec{a}_1 \hat{n} \cdot \vec{v}_2 \hat{n} \cdot \vec{v}_1 - \frac{13}{4} \hat{n} \times \vec{S}_1 \cdot \vec{v}_1 \vec{a}_1 \cdot \vec{v}_2 \hat{n} \cdot \vec{v}_1 + \\
& \quad \frac{15}{8} \hat{n} \times \vec{S}_1 \cdot \vec{v}_1 \vec{v}_1 \cdot \vec{a}_1 \hat{n} \cdot \vec{v}_1 + \frac{13}{24} \hat{n} \times \vec{S}_1 \cdot \vec{v}_1 \vec{v}_1 \cdot \vec{a}_2 \hat{n} \cdot \vec{v}_1 + 2 \hat{n} \times \vec{S}_1 \cdot \vec{v}_1 \vec{v}_1 \cdot \vec{v}_1 \hat{n} \cdot \vec{v}_1 + \frac{3}{2} \hat{n} \times \vec{S}_1 \cdot \vec{a}_1 \vec{v}_1 \cdot \vec{v}_1 \hat{n} \cdot \vec{v}_1 - \\
& \quad \frac{37}{6} \hat{n} \times \vec{S}_1 \cdot \vec{v}_1 \vec{v}_1 \cdot \vec{v}_2 \hat{n} \cdot \vec{v}_1 - \frac{11}{4} \hat{n} \times \vec{S}_1 \cdot \vec{a}_1 \vec{v}_1 \cdot \vec{v}_2 \hat{n} \cdot \vec{v}_1 + \hat{n} \times \vec{S}_1 \cdot \vec{v}_1 \vec{v}_2 \cdot \vec{v}_2 \hat{n} \cdot \vec{v}_1 + \frac{7}{12} \hat{n} \times \vec{S}_1 \cdot \vec{a}_1 \vec{v}_2 \cdot \vec{v}_2 \hat{n} \cdot \vec{v}_1 + \\
& \quad \frac{1}{3} \vec{S}_1 \times \vec{v}_1 \cdot \vec{a}_1 (\hat{n} \cdot \vec{v}_2)^2 - \frac{11}{3} \hat{n} \times \vec{S}_1 \cdot \vec{v}_1 \hat{n} \cdot \vec{a}_1 (\hat{n} \cdot \vec{v}_2)^2 + \frac{11}{6} \vec{S}_1 \times \vec{v}_1 \cdot \vec{v}_2 \hat{n} \cdot \vec{a}_1 \hat{n} \cdot \vec{v}_2 - \frac{11}{12} \vec{S}_1 \times \vec{v}_1 \cdot \vec{v}_2 \vec{a}_1 \cdot \vec{v}_2 + \\
& \quad \frac{11}{6} \hat{n} \times \vec{S}_1 \cdot \vec{v}_1 \hat{n} \cdot \vec{v}_2 \vec{a}_1 \cdot \vec{v}_2 + \frac{1}{2} \vec{S}_1 \times \vec{v}_1 \cdot \vec{v}_2 \vec{v}_1 \cdot \vec{a}_1 - \hat{n} \times \vec{S}_1 \cdot \vec{v}_1 \hat{n} \cdot \vec{v}_2 \vec{v}_1 \cdot \vec{a}_1 + \frac{5}{12} \vec{S}_1 \times \vec{v}_1 \cdot \vec{v}_2 \vec{v}_1 \cdot \vec{v}_1 + \\
& \quad \frac{1}{8} \vec{S}_1 \times \vec{a}_1 \cdot \vec{v}_2 \vec{v}_1 \cdot \vec{v}_1 + \frac{9}{16} \vec{S}_1 \times \vec{v}_1 \cdot \vec{a}_1 \vec{v}_1 \cdot \vec{v}_1 + \frac{7}{48} \vec{S}_1 \times \vec{v}_1 \cdot \vec{a}_2 \vec{v}_1 \cdot \vec{v}_1 + \frac{3}{8} \hat{n} \times \vec{S}_1 \cdot \vec{v}_1 \hat{n} \cdot \vec{a}_1 \vec{v}_1 \cdot \vec{v}_1 - \\
& \quad \frac{7}{24} \hat{n} \times \vec{S}_1 \cdot \vec{v}_1 \hat{n} \cdot \vec{a}_2 \vec{v}_1 \cdot \vec{v}_1 - \frac{5}{6} \hat{n} \times \vec{S}_1 \cdot \vec{v}_1 \hat{n} \cdot \vec{v}_2 \vec{v}_1 \cdot \vec{v}_1 - \frac{1}{4} \hat{n} \times \vec{S}_1 \cdot \vec{a}_1 \hat{n} \cdot \vec{v}_2 \vec{v}_1 \cdot \vec{v}_1 - \vec{S}_1 \times \vec{v}_1 \cdot \vec{v}_2 \vec{v}_1 \cdot \vec{v}_2 - \\
& \quad \frac{7}{12} \vec{S}_1 \times \vec{a}_1 \cdot \vec{v}_2 \vec{v}_1 \cdot \vec{v}_2 + \frac{1}{4} \vec{S}_1 \times \vec{v}_1 \cdot \vec{a}_1 \vec{v}_1 \cdot \vec{v}_2 - \frac{13}{4} \hat{n} \times \vec{S}_1 \cdot \vec{v}_1 \hat{n} \cdot \vec{a}_1 \vec{v}_1 \cdot \vec{v}_2 + 2 \hat{n} \times \vec{S}_1 \cdot \vec{v}_1 \hat{n} \cdot \vec{v}_2 \vec{v}_1 \cdot \vec{v}_2 + \\
& \quad \frac{7}{6} \hat{n} \times \vec{S}_1 \cdot \vec{a}_1 \hat{n} \cdot \vec{v}_2 \vec{v}_1 \cdot \vec{v}_2 - \frac{1}{6} \vec{S}_1 \times \vec{v}_1 \cdot \vec{a}_1 \vec{v}_2 \cdot \vec{v}_2 + \frac{11}{12} \hat{n} \times \vec{S}_1 \cdot \vec{v}_1 \hat{n} \cdot \vec{a}_1 \vec{v}_2 \cdot \vec{v}_2 \Big) m_1 m_2 G^2 + \\
& \quad \frac{1}{r^3} \left( -\frac{119}{32} \hat{n} \times \vec{S}_1 \cdot \vec{v}_1 (\hat{n} \cdot \vec{v}_1)^4 - \frac{3}{2} \vec{S}_1 \times \vec{v}_1 \cdot \vec{v}_2 (\hat{n} \cdot \vec{v}_1)^3 + 9 \hat{n} \times \vec{S}_1 \cdot \vec{v}_1 \hat{n} \cdot \vec{v}_2 (\hat{n} \cdot \vec{v}_1)^3 - \right. \\
& \quad \frac{13}{2} \hat{n} \times \vec{S}_1 \cdot \vec{v}_1 (\hat{n} \cdot \vec{v}_2)^2 (\hat{n} \cdot \vec{v}_1)^2 + \frac{13}{6} \vec{S}_1 \times \vec{v}_1 \cdot \vec{v}_2 \hat{n} \cdot \vec{v}_2 (\hat{n} \cdot \vec{v}_1)^2 - \frac{47}{16} \hat{n} \times \vec{S}_1 \cdot \vec{v}_1 \vec{v}_1 \cdot \vec{v}_1 (\hat{n} \cdot \vec{v}_1)^2 - \\
& \quad \frac{9}{2} \hat{n} \times \vec{S}_1 \cdot \vec{v}_1 \vec{v}_1 \cdot \vec{v}_2 (\hat{n} \cdot \vec{v}_1)^2 + \frac{13}{12} \hat{n} \times \vec{S}_1 \cdot \vec{v}_1 \vec{v}_2 \cdot \vec{v}_2 (\hat{n} \cdot \vec{v}_1)^2 - \frac{3}{2} \vec{S}_1 \times \vec{v}_1 \cdot \vec{v}_2 \vec{v}_1 \cdot \vec{v}_1 \hat{n} \cdot \vec{v}_1 + \\
& \quad 6 \hat{n} \times \vec{S}_1 \cdot \vec{v}_1 \hat{n} \cdot \vec{v}_2 \vec{v}_1 \cdot \vec{v}_1 \hat{n} \cdot \vec{v}_1 - \frac{13}{12} \vec{S}_1 \times \vec{v}_1 \cdot \vec{v}_2 \vec{v}_1 \cdot \vec{v}_2 \hat{n} \cdot \vec{v}_1 + \frac{13}{3} \hat{n} \times \vec{S}_1 \cdot \vec{v}_1 \hat{n} \cdot \vec{v}_2 \vec{v}_1 \cdot \vec{v}_2 \hat{n} \cdot \vec{v}_1 + \\
& \quad \frac{29}{32} \hat{n} \times \vec{S}_1 \cdot \vec{v}_1 (\vec{v}_1 \cdot \vec{v}_1)^2 - \frac{13}{24} \hat{n} \times \vec{S}_1 \cdot \vec{v}_1 (\vec{v}_1 \cdot \vec{v}_2)^2 - \frac{7}{6} \hat{n} \times \vec{S}_1 \cdot \vec{v}_1 (\hat{n} \cdot \vec{v}_2)^2 \vec{v}_1 \cdot \vec{v}_1 + \\
& \quad \left. \frac{7}{12} \vec{S}_1 \times \vec{v}_1 \cdot \vec{v}_2 \hat{n} \cdot \vec{v}_2 \vec{v}_1 \cdot \vec{v}_1 - \frac{3}{2} \hat{n} \times \vec{S}_1 \cdot \vec{v}_1 \vec{v}_1 \cdot \vec{v}_1 \vec{v}_1 \cdot \vec{v}_2 + \frac{7}{24} \hat{n} \times \vec{S}_1 \cdot \vec{v}_1 \vec{v}_1 \cdot \vec{v}_1 \vec{v}_2 \cdot \vec{v}_2 \right) m_1 m_2 G^2 + \\
& \quad m_1 m_2 \left( -\frac{1}{6} \log \left( \frac{r}{R_\theta} \right) \vec{S}_1 \times \vec{a}_1 \cdot \vec{a}_2 + \frac{17}{72} \vec{S}_1 \times \vec{a}_1 \cdot \vec{a}_2 + \frac{17}{144} \vec{S}_1 \times \vec{v}_1 \cdot \vec{a}_1 + \frac{17}{144} \vec{S}_1 \times \vec{v}_1 \cdot \vec{a}_2 + \frac{17}{144} \vec{S}_1 \times \vec{a}_1 \cdot \vec{a}_2 - \right. \\
& \quad \frac{17}{144} \vec{S}_1 \times \vec{a}_1 \cdot \vec{a}_1 + \frac{5}{24} \hat{n} \times \vec{S}_1 \cdot \vec{a}_1 \hat{n} \cdot \vec{a}_1 + \frac{2}{3} \hat{n} \times \vec{S}_1 \cdot \vec{a}_1 \hat{n} \cdot \vec{a}_1 + \frac{1}{8} \hat{n} \times \vec{S}_1 \cdot \vec{v}_1 \hat{n} \cdot \vec{a}_1 + \frac{1}{8} \hat{n} \times \vec{S}_1 \cdot \vec{a}_1 \hat{n} \cdot \vec{a}_1 - \\
& \quad \frac{1}{6} \hat{n} \times \vec{S}_1 \cdot \vec{a}_1 \hat{n} \cdot \vec{a}_2 - \frac{1}{12} \hat{n} \times \vec{S}_1 \cdot \vec{v}_1 \hat{n} \cdot \vec{a}_2 - \frac{1}{12} \hat{n} \times \vec{S}_1 \cdot \vec{a}_1 \hat{n} \cdot \vec{a}_2 + \frac{5}{24} \hat{n} \times \vec{S}_1 \cdot \vec{a}_1 \hat{n} \cdot \vec{v}_1 - \\
& \quad \frac{1}{12} \vec{S}_1 \times \vec{v}_1 \cdot \vec{a}_1 \log \left( \frac{r}{R_\theta} \right) - \frac{1}{12} \vec{S}_1 \times \vec{v}_1 \cdot \vec{a}_2 \log \left( \frac{r}{R_\theta} \right) - \frac{1}{12} \vec{S}_1 \times \vec{a}_1 \cdot \vec{a}_2 \log \left( \frac{r}{R_\theta} \right) + \frac{1}{12} \vec{S}_1 \times \vec{a}_1 \cdot \vec{a}_1 \log \left( \frac{r}{R_\theta} \right) + \\
& \quad \left. \frac{1}{\epsilon_d} \left( \frac{1}{12} \vec{S}_1 \times \vec{a}_1 \cdot \vec{a}_2 + \frac{1}{24} \vec{S}_1 \times \vec{v}_1 \cdot \vec{a}_1 + \frac{1}{24} \vec{S}_1 \times \vec{v}_1 \cdot \vec{a}_2 + \frac{1}{24} \vec{S}_1 \times \vec{a}_1 \cdot \vec{a}_2 - \frac{1}{24} \vec{S}_1 \times \vec{a}_1 \cdot \vec{a}_1 \right) \right) G^2 \Big\}
\end{aligned}$$

{DiagSet[2, 2, 130],

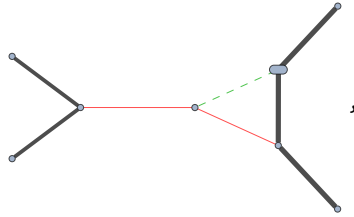

,

$$\frac{1}{r} \left( 12 \hat{n} \times \vec{S}_1 \cdot \vec{v}_1 \vec{v}_1 \cdot \vec{a}_1 + 12 \hat{n} \times \vec{S}_1 \cdot \vec{a}_1 \vec{v}_1 \cdot \vec{a}_1 - 6 \hat{n} \times \vec{S}_1 \cdot \vec{v}_1 \vec{v}_2 \cdot \vec{a}_2 - 6 \hat{n} \times \vec{S}_1 \cdot \vec{a}_1 \vec{v}_2 \cdot \vec{a}_2 \right) m_1 m_2 G^2 + \frac{1}{r^2} \left( 4 \vec{S}_1 \times \vec{v}_1 \cdot \vec{a}_1 (\hat{n} \cdot \vec{v}_1)^2 + 4 \vec{S}_1 \times \vec{v}_1 \cdot \vec{a}_1 \hat{n} \cdot \vec{v}_2 \hat{n} \cdot \vec{v}_1 - 16 \hat{n} \times \vec{S}_1 \cdot \vec{v}_1 \vec{v}_1 \cdot \vec{a}_1 \hat{n} \cdot \vec{v}_1 - 8 \hat{n} \times \vec{S}_1 \cdot \vec{v}_1 \vec{v}_1 \cdot \vec{v}_1 \hat{n} \cdot \vec{v}_1 - 8 \hat{n} \times \vec{S}_1 \cdot \vec{a}_1 \vec{v}_1 \cdot \vec{v}_1 \hat{n} \cdot \vec{v}_1 + 3 \hat{n} \times \vec{S}_1 \cdot \vec{v}_1 \vec{v}_2 \cdot \vec{a}_2 \hat{n} \cdot \vec{v}_1 - 6 \hat{n} \times \vec{S}_1 \cdot \vec{v}_1 \vec{v}_2 \cdot \vec{v}_2 \hat{n} \cdot \vec{v}_1 - 6 \hat{n} \times \vec{S}_1 \cdot \vec{a}_1 \vec{v}_2 \cdot \vec{v}_2 \hat{n} \cdot \vec{v}_1 + 2 \vec{S}_1 \times \vec{v}_1 \cdot \vec{v}_2 \vec{v}_1 \cdot \vec{a}_1 - 4 \hat{n} \times \vec{S}_1 \cdot \vec{v}_1 \hat{n} \cdot \vec{v}_2 \vec{v}_1 \cdot \vec{a}_1 + 4 \vec{S}_1 \times \vec{v}_1 \cdot \vec{v}_2 \vec{v}_1 \cdot \vec{v}_1 + 4 \vec{S}_1 \times \vec{a}_1 \cdot \vec{v}_2 \vec{v}_1 \cdot \vec{v}_1 - 6 \vec{S}_1 \times \vec{v}_1 \cdot \vec{a}_1 \vec{v}_1 \cdot \vec{v}_1 - 8 \hat{n} \times \vec{S}_1 \cdot \vec{v}_1 \hat{n} \cdot \vec{v}_2 \vec{v}_1 \cdot \vec{v}_1 - 8 \hat{n} \times \vec{S}_1 \cdot \vec{a}_1 \hat{n} \cdot \vec{v}_2 \vec{v}_1 \cdot \vec{v}_1 - 2 \vec{S}_1 \times \vec{v}_1 \cdot \vec{a}_1 \vec{v}_1 \cdot \vec{v}_2 + 3 \vec{S}_1 \times \vec{v}_1 \cdot \vec{v}_2 \vec{v}_2 \cdot \vec{v}_2 + 3 \vec{S}_1 \times \vec{a}_1 \cdot \vec{v}_2 \vec{v}_2 \cdot \vec{v}_2 - 3 \vec{S}_1 \times \vec{v}_1 \cdot \vec{a}_1 \vec{v}_2 \cdot \vec{v}_2 - 6 \hat{n} \times \vec{S}_1 \cdot \vec{v}_1 \hat{n} \cdot \vec{v}_2 \vec{v}_2 \cdot \vec{v}_2 - 6 \hat{n} \times \vec{S}_1 \cdot \vec{a}_1 \hat{n} \cdot \vec{v}_2 \vec{v}_2 \cdot \vec{v}_2 \right) m_1 m_2 G^2 + \frac{1}{r^3} \left( 8 \hat{n} \times \vec{S}_1 \cdot \vec{v}_1 \vec{v}_1 \cdot \vec{v}_1 (\hat{n} \cdot \vec{v}_1)^2 + 6 \hat{n} \times \vec{S}_1 \cdot \vec{v}_1 \vec{v}_2 \cdot \vec{v}_2 (\hat{n} \cdot \vec{v}_1)^2 - 2 \vec{S}_1 \times \vec{v}_1 \cdot \vec{v}_2 \vec{v}_1 \cdot \vec{v}_1 \hat{n} \cdot \vec{v}_1 + 8 \hat{n} \times \vec{S}_1 \cdot \vec{v}_1 \hat{n} \cdot \vec{v}_2 \vec{v}_1 \cdot \vec{v}_1 \hat{n} \cdot \vec{v}_1 - \frac{3}{2} \vec{S}_1 \times \vec{v}_1 \cdot \vec{v}_2 \vec{v}_2 \cdot \vec{v}_2 \hat{n} \cdot \vec{v}_1 + 6 \hat{n} \times \vec{S}_1 \cdot \vec{v}_1 \hat{n} \cdot \vec{v}_2 \vec{v}_2 \cdot \vec{v}_2 \hat{n} \cdot \vec{v}_1 - 2 \hat{n} \times \vec{S}_1 \cdot \vec{v}_1 (\vec{v}_1 \cdot \vec{v}_1)^2 + \frac{7}{16} \hat{n} \times \vec{S}_1 \cdot \vec{v}_1 (\vec{v}_2 \cdot \vec{v}_2)^2 - 2 \hat{n} \times \vec{S}_1 \cdot \vec{v}_1 \vec{v}_1 \cdot \vec{v}_1 \vec{v}_1 \cdot \vec{v}_2 - \frac{3}{4} \hat{n} \times \vec{S}_1 \cdot \vec{v}_1 \vec{v}_1 \cdot \vec{v}_1 \vec{v}_2 \cdot \vec{v}_2 - \frac{3}{2} \hat{n} \times \vec{S}_1 \cdot \vec{v}_1 \vec{v}_1 \cdot \vec{v}_2 \vec{v}_2 \cdot \vec{v}_2 \right) m_1 m_2 G^2 \Big\}$$

{DiagSet[2, 2, 131],

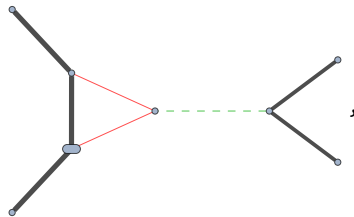

,

$$\frac{1}{r^2} G^2 m_1 m_2 \left( -4 \hat{n} \cdot \vec{v}_1 \hat{n} \cdot \vec{v}_2 \vec{S}_1 \times \vec{v}_1 \cdot \vec{a}_1 + 20 \vec{v}_1 \cdot \vec{a}_1 \hat{n} \cdot \vec{v}_2 \hat{n} \times \vec{S}_1 \cdot \vec{v}_1 + 4 \vec{v}_1 \cdot \vec{v}_1 \hat{n} \cdot \vec{v}_2 \hat{n} \times \vec{S}_1 \cdot \vec{a}_1 + \vec{v}_2 \cdot \vec{v}_2 \hat{n} \cdot \vec{v}_2 \hat{n} \times \vec{S}_1 \cdot \vec{a}_1 - 8 \vec{v}_1 \cdot \vec{a}_1 \vec{S}_1 \times \vec{v}_1 \cdot \vec{v}_2 - 4 \vec{v}_1 \cdot \vec{v}_1 \vec{S}_1 \times \vec{a}_1 \cdot \vec{v}_2 + 4 \vec{v}_1 \cdot \vec{v}_2 \vec{S}_1 \times \vec{v}_1 \cdot \vec{a}_1 - \vec{v}_2 \cdot \vec{v}_2 \vec{S}_1 \times \vec{a}_1 \cdot \vec{v}_2 + 4 \vec{v}_1 \cdot \vec{v}_1 \hat{n} \cdot \vec{v}_2 \hat{n} \times \vec{S}_1 \cdot \vec{v}_1 + \vec{v}_2 \cdot \vec{v}_2 \hat{n} \cdot \vec{v}_2 \hat{n} \times \vec{S}_1 \cdot \vec{v}_1 - 4 \vec{v}_1 \cdot \vec{v}_1 \vec{S}_1 \times \vec{v}_1 \cdot \vec{v}_2 - \vec{v}_2 \cdot \vec{v}_2 \vec{S}_1 \times \vec{v}_1 \cdot \vec{v}_2 \right) + \frac{G^2 m_1 m_2 \left( 4 \hat{n} \cdot \vec{v}_2 \vec{S}_1 \times \vec{v}_1 \cdot \vec{a}_1 + 4 \hat{n} \cdot \vec{v}_2 \vec{S}_1 \times \vec{v}_1 \cdot \vec{a}_1 \right)}{r} + \frac{1}{r^3} G^2 m_1 m_2 \left( 4 \vec{v}_1 \cdot \vec{v}_1 \hat{n} \cdot \vec{v}_1 \vec{S}_1 \times \vec{v}_1 \cdot \vec{v}_2 - 16 \vec{v}_1 \cdot \vec{v}_1 \hat{n} \cdot \vec{v}_1 \hat{n} \cdot \vec{v}_2 \hat{n} \times \vec{S}_1 \cdot \vec{v}_1 + 8 \vec{v}_1 \cdot \vec{v}_2 \vec{v}_1 \cdot \vec{v}_1 \hat{n} \times \vec{S}_1 \cdot \vec{v}_1 + \vec{v}_2 \cdot \vec{v}_2 \hat{n} \cdot \vec{v}_1 \vec{S}_1 \times \vec{v}_1 \cdot \vec{v}_2 - 4 \vec{v}_2 \cdot \vec{v}_2 \hat{n} \cdot \vec{v}_1 \hat{n} \cdot \vec{v}_2 \hat{n} \times \vec{S}_1 \cdot \vec{v}_1 + 2 \vec{v}_1 \cdot \vec{v}_2 \vec{v}_2 \cdot \vec{v}_2 \hat{n} \times \vec{S}_1 \cdot \vec{v}_1 \right) \Big\}$$

{DiagSet[2, 2, 132],

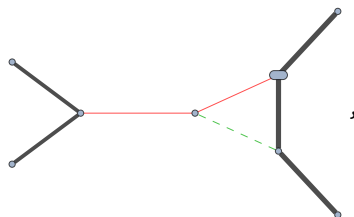

,

$$\frac{1}{r^2} G^2 m_1 m_2 \left( 8 (\hat{n} \cdot \vec{v}_1)^2 \vec{S}_1 \times \vec{v}_1 \cdot \vec{a}_1 + 8 \hat{n} \cdot \vec{v}_2 \hat{n} \cdot \vec{v}_1 \vec{S}_1 \times \vec{v}_1 \cdot \vec{a}_1 - 8 \vec{v}_1 \cdot \vec{a}_1 \hat{n} \cdot \vec{v}_1 \hat{n} \times \vec{S}_1 \cdot \vec{v}_1 - \right.$$

$$\begin{aligned}
 & 8 \vec{v}_1 \cdot \vec{v}_1 \hat{n} \cdot \vec{v}_1 \hat{n} \times \vec{S}_1 \cdot \vec{a}_1 + 18 \vec{v}_2 \cdot \vec{a}_2 \hat{n} \cdot \vec{v}_1 \hat{n} \times \vec{S}_1 \cdot \vec{v}_1 - 12 \vec{v}_2 \cdot \vec{v}_2 \hat{n} \cdot \vec{v}_1 \hat{n} \times \vec{S}_1 \cdot \vec{a}_1 - 8 \vec{v}_1 \cdot \vec{v}_1 \vec{S}_1 \times \vec{v}_1 \cdot \vec{a}_1 - \\
 & 4 \vec{v}_1 \cdot \vec{v}_2 \vec{S}_1 \times \vec{v}_1 \cdot \vec{a}_1 - 6 \vec{v}_2 \cdot \vec{v}_2 \vec{S}_1 \times \vec{v}_1 \cdot \vec{a}_1 - 8 \vec{v}_1 \cdot \vec{v}_1 \hat{n} \cdot \vec{v}_1 \hat{n} \times \vec{S}_1 \cdot \vec{v}_1 - 12 \vec{v}_2 \cdot \vec{v}_2 \hat{n} \cdot \vec{v}_1 \hat{n} \times \vec{S}_1 \cdot \vec{v}_1 \Big) + \\
 & \frac{G^2 m_1 m_2 \left( -8 \hat{n} \cdot \vec{v}_1 \vec{S}_1 \times \vec{v}_1 \cdot \vec{a}_1 - 8 \hat{n} \cdot \vec{v}_1 \vec{S}_1 \times \vec{v}_1 \cdot \frac{1}{a_1} \right)}{r} + \frac{1}{r^3} \\
 & G^2 m_1 m_2 \left( 24 \vec{v}_1 \cdot \vec{v}_1 (\hat{n} \cdot \vec{v}_1)^2 \hat{n} \times \vec{S}_1 \cdot \vec{v}_1 + 36 \vec{v}_2 \cdot \vec{v}_2 (\hat{n} \cdot \vec{v}_1)^2 \hat{n} \times \vec{S}_1 \cdot \vec{v}_1 - 6 \vec{v}_1 \cdot \vec{v}_1 \hat{n} \cdot \vec{v}_1 \vec{S}_1 \times \vec{v}_1 \cdot \vec{v}_2 + \right. \\
 & 24 \vec{v}_1 \cdot \vec{v}_1 \hat{n} \cdot \vec{v}_2 \hat{n} \cdot \vec{v}_1 \hat{n} \times \vec{S}_1 \cdot \vec{v}_1 - 9 \vec{v}_2 \cdot \vec{v}_2 \hat{n} \cdot \vec{v}_1 \vec{S}_1 \times \vec{v}_1 \cdot \vec{v}_2 + 36 \vec{v}_2 \cdot \vec{v}_2 \hat{n} \cdot \vec{v}_2 \hat{n} \cdot \vec{v}_1 \hat{n} \times \vec{S}_1 \cdot \vec{v}_1 - \\
 & \left. 6 (\vec{v}_1 \cdot \vec{v}_1)^2 \hat{n} \times \vec{S}_1 \cdot \vec{v}_1 - 6 \vec{v}_1 \cdot \vec{v}_1 \vec{v}_1 \cdot \vec{v}_2 \hat{n} \times \vec{S}_1 \cdot \vec{v}_1 - 9 \vec{v}_1 \cdot \vec{v}_1 \vec{v}_2 \cdot \vec{v}_2 \hat{n} \times \vec{S}_1 \cdot \vec{v}_1 - 9 \vec{v}_1 \cdot \vec{v}_2 \vec{v}_2 \cdot \vec{v}_2 \hat{n} \times \vec{S}_1 \cdot \vec{v}_1 \right) \Big\}
 \end{aligned}$$

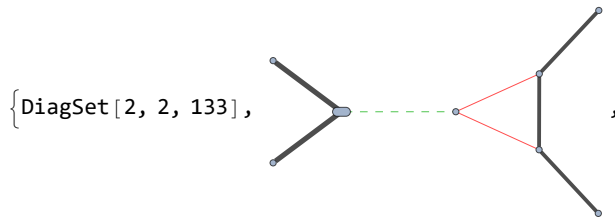

$$\begin{aligned}
 & \frac{1}{r^2} G^2 m_2^2 \left( \hat{n} \cdot \vec{v}_1 \hat{n} \cdot \vec{v}_2 \left( -(\vec{a}_1 \times \vec{S}_1 \cdot \vec{v}_1) \right) + \vec{a}_1 \cdot \vec{v}_1 \hat{n} \cdot \vec{v}_2 \hat{n} \times \vec{S}_1 \cdot \vec{v}_1 - \frac{1}{2} \vec{v}_1 \cdot \vec{v}_1 \hat{n} \cdot \vec{v}_2 \hat{n} \times \vec{a}_1 \cdot \vec{S}_1 - 3 \vec{v}_2 \cdot \vec{v}_2 \hat{n} \cdot \vec{v}_2 \hat{n} \times \vec{a}_1 \cdot \vec{S}_1 - \right. \\
 & 12 \vec{a}_2 \cdot \vec{v}_2 \hat{n} \cdot \vec{v}_1 \hat{n} \times \vec{S}_1 \cdot \vec{v}_1 - \vec{a}_1 \cdot \vec{v}_1 \vec{S}_1 \times \vec{v}_1 \cdot \vec{v}_2 + \frac{1}{2} \vec{v}_1 \cdot \vec{v}_1 \vec{a}_1 \times \vec{S}_1 \cdot \vec{v}_2 + \vec{v}_1 \cdot \vec{v}_2 \vec{a}_1 \times \vec{S}_1 \cdot \vec{v}_1 + 3 \vec{v}_2 \cdot \vec{v}_2 \vec{a}_1 \times \vec{S}_1 \cdot \vec{v}_2 + \\
 & \left. \frac{1}{2} \vec{v}_1 \cdot \vec{v}_1 \hat{n} \cdot \vec{v}_2 \hat{n} \times \vec{S}_1 \cdot \vec{v}_1 + 3 \vec{v}_2 \cdot \vec{v}_2 \hat{n} \cdot \vec{v}_2 \hat{n} \times \vec{S}_1 \cdot \vec{v}_1 - \frac{1}{2} \vec{v}_1 \cdot \vec{v}_1 \vec{S}_1 \times \vec{v}_1 \cdot \vec{v}_2 - 3 \vec{v}_2 \cdot \vec{v}_2 \vec{S}_1 \times \vec{v}_1 \cdot \vec{v}_2 \right) + \\
 & \frac{G^2 m_2^2 \left( 6 \vec{a}_2 \cdot \vec{v}_2 \hat{n} \times \vec{S}_1 \cdot \vec{v}_1 - 6 \vec{a}_2 \cdot \vec{v}_2 \hat{n} \times \vec{a}_1 \cdot \vec{S}_1 \right)}{r} + \frac{1}{r^3} G^2 m_2^2 \\
 & \left( 2 (\vec{v}_2 \cdot \vec{v}_2)^2 \hat{n} \times \vec{S}_1 \cdot \vec{v}_2 + \frac{15}{4} \vec{v}_2 \cdot \vec{v}_2 \hat{n} \cdot \vec{v}_1 \vec{S}_1 \times \vec{v}_1 \cdot \vec{v}_2 - 12 \vec{v}_2 \cdot \vec{v}_2 \hat{n} \cdot \vec{v}_1 \hat{n} \cdot \vec{v}_2 \hat{n} \times \vec{S}_1 \cdot \vec{v}_1 + \frac{21}{4} \vec{v}_1 \cdot \vec{v}_2 \vec{v}_2 \cdot \vec{v}_2 \hat{n} \times \vec{S}_1 \cdot \vec{v}_1 + \right. \\
 & \left. \frac{9}{16} \vec{v}_1 \cdot \vec{v}_1 \hat{n} \cdot \vec{v}_1 \vec{S}_1 \times \vec{v}_1 \cdot \vec{v}_2 - 2 \vec{v}_1 \cdot \vec{v}_1 \hat{n} \cdot \vec{v}_1 \hat{n} \cdot \vec{v}_2 \hat{n} \times \vec{S}_1 \cdot \vec{v}_1 + \frac{15}{16} \vec{v}_1 \cdot \vec{v}_1 \vec{v}_1 \cdot \vec{v}_2 \hat{n} \times \vec{S}_1 \cdot \vec{v}_1 \right) \Big\}
 \end{aligned}$$

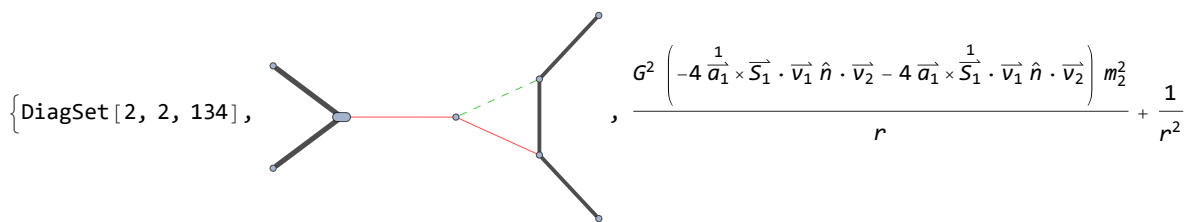

$$\begin{aligned}
 & G^2 \left( 8 \vec{a}_1 \times \vec{S}_1 \cdot \vec{v}_1 (\hat{n} \cdot \vec{v}_2)^2 + 8 \vec{a}_1 \times \vec{S}_1 \cdot \vec{v}_1 \hat{n} \cdot \vec{v}_1 \hat{n} \cdot \vec{v}_2 - 8 \hat{n} \times \vec{S}_1 \cdot \vec{v}_1 \vec{a}_1 \cdot \vec{v}_1 \hat{n} \cdot \vec{v}_2 + 48 \hat{n} \times \vec{S}_1 \cdot \vec{v}_1 \vec{a}_2 \cdot \vec{v}_2 \hat{n} \cdot \vec{v}_2 - \right. \\
 & 4 \hat{n} \times \vec{S}_1 \cdot \vec{v}_1 \vec{v}_1 \cdot \vec{v}_1 \hat{n} \cdot \vec{v}_2 + 4 \hat{n} \times \vec{a}_1 \cdot \vec{S}_1 \vec{v}_1 \cdot \vec{v}_1 \hat{n} \cdot \vec{v}_2 - 16 \hat{n} \times \vec{S}_1 \cdot \vec{v}_1 \vec{v}_2 \cdot \vec{v}_2 \hat{n} \cdot \vec{v}_2 + 16 \hat{n} \times \vec{a}_1 \cdot \vec{S}_1 \vec{v}_2 \cdot \vec{v}_2 \hat{n} \cdot \vec{v}_2 + \\
 & 4 \vec{S}_1 \times \vec{v}_1 \cdot \vec{v}_2 \vec{a}_1 \cdot \vec{v}_1 - 24 \vec{S}_1 \times \vec{v}_1 \cdot \vec{v}_2 \vec{a}_2 \cdot \vec{v}_2 + 2 \vec{S}_1 \times \vec{v}_1 \cdot \vec{v}_2 \vec{v}_1 \cdot \vec{v}_1 - 2 \vec{a}_1 \times \vec{S}_1 \cdot \vec{v}_2 \vec{v}_1 \cdot \vec{v}_1 - \\
 & \left. 4 \vec{a}_1 \times \vec{S}_1 \cdot \vec{v}_1 \vec{v}_1 \cdot \vec{v}_2 + 8 \vec{S}_1 \times \vec{v}_1 \cdot \vec{v}_2 \vec{v}_2 \cdot \vec{v}_2 - 4 \vec{a}_1 \times \vec{S}_1 \cdot \vec{v}_1 \vec{v}_2 \cdot \vec{v}_2 - 8 \vec{a}_1 \times \vec{S}_1 \cdot \vec{v}_2 \vec{v}_2 \cdot \vec{v}_2 \right) m_2^2 + \\
 & \frac{1}{r^3} G^2 \left( 16 \hat{n} \times \vec{S}_1 \cdot \vec{v}_1 \vec{v}_1 \cdot \vec{v}_1 (\hat{n} \cdot \vec{v}_2)^2 + 64 \hat{n} \times \vec{S}_1 \cdot \vec{v}_1 \vec{v}_2 \cdot \vec{v}_2 (\hat{n} \cdot \vec{v}_2)^2 - 8 \vec{S}_1 \times \vec{v}_1 \cdot \vec{v}_2 \vec{v}_1 \cdot \vec{v}_1 \hat{n} \cdot \vec{v}_2 + \right. \\
 & 16 \hat{n} \times \vec{S}_1 \cdot \vec{v}_1 \hat{n} \cdot \vec{v}_1 \vec{v}_1 \cdot \vec{v}_1 \hat{n} \cdot \vec{v}_2 - 32 \vec{S}_1 \times \vec{v}_1 \cdot \vec{v}_2 \vec{v}_2 \cdot \vec{v}_2 \hat{n} \cdot \vec{v}_2 + 64 \hat{n} \times \vec{S}_1 \cdot \vec{v}_1 \hat{n} \cdot \vec{v}_1 \vec{v}_2 \cdot \vec{v}_2 \hat{n} \cdot \vec{v}_2 - \\
 & 16 \hat{n} \times \vec{S}_1 \cdot \vec{v}_1 (\vec{v}_2 \cdot \vec{v}_2)^2 - 4 \vec{S}_1 \times \vec{v}_1 \cdot \vec{v}_2 \hat{n} \cdot \vec{v}_1 \vec{v}_1 \cdot \vec{v}_1 - 4 \hat{n} \times \vec{S}_1 \cdot \vec{v}_1 \vec{v}_1 \cdot \vec{v}_1 \vec{v}_1 \cdot \vec{v}_2 - \\
 & \left. 16 \vec{S}_1 \times \vec{v}_1 \cdot \vec{v}_2 \hat{n} \cdot \vec{v}_1 \vec{v}_2 \cdot \vec{v}_2 - 4 \hat{n} \times \vec{S}_1 \cdot \vec{v}_1 \vec{v}_1 \cdot \vec{v}_1 \vec{v}_2 \cdot \vec{v}_2 - 16 \hat{n} \times \vec{S}_1 \cdot \vec{v}_1 \vec{v}_1 \cdot \vec{v}_2 \vec{v}_2 \cdot \vec{v}_2 \right) m_2^2 \Big\}
 \end{aligned}$$

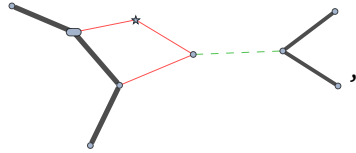

Printed by Wolfram Mathematica Student Edition

$$\left. \frac{4}{3} \vec{S}_1 \times \vec{a}_1 \cdot \vec{a}_2 \log \left( \frac{r}{R_\theta} \right) + \frac{\frac{4}{3} \vec{S}_1 \times \vec{a}_1 \cdot \vec{a}_2 + \frac{2}{3} \vec{S}_1 \times \vec{v}_1 \cdot \vec{a}_2 + \frac{2}{3} \vec{S}_1 \times \vec{a}_1 \cdot \vec{a}_2}{\epsilon_d} \right\} G^2 \}$$

$\{\text{DiagSet}[2, 2, 136],$

[illegible]

$$\begin{aligned}
& 4 \hat{n} \times \vec{S}_1 \cdot \vec{v}_1 \vec{v}_1 \cdot \vec{v}_2 (\hat{n} \cdot \vec{v}_1)^2 + \frac{4}{3} \hat{n} \times \vec{S}_1 \cdot \vec{v}_1 \vec{v}_2 \cdot \vec{v}_2 (\hat{n} \cdot \vec{v}_1)^2 - \frac{1}{2} \vec{S}_1 \times \vec{v}_1 \cdot \vec{v}_2 \vec{v}_1 \cdot \vec{v}_1 \hat{n} \cdot \vec{v}_1 + \\
& 2 \hat{n} \times \vec{S}_1 \cdot \vec{v}_1 \hat{n} \cdot \vec{v}_2 \vec{v}_1 \cdot \vec{v}_1 \hat{n} \cdot \vec{v}_1 - \frac{4}{3} \vec{S}_1 \times \vec{v}_1 \cdot \vec{v}_2 \vec{v}_1 \cdot \vec{v}_2 \hat{n} \cdot \vec{v}_1 + \frac{16}{3} \hat{n} \times \vec{S}_1 \cdot \vec{v}_1 \hat{n} \cdot \vec{v}_2 \vec{v}_1 \cdot \vec{v}_2 \hat{n} \cdot \vec{v}_1 + \\
& \frac{3}{4} \vec{S}_1 \times \vec{v}_1 \cdot \vec{v}_2 \vec{v}_2 \cdot \vec{v}_2 \hat{n} \cdot \vec{v}_1 - 3 \hat{n} \times \vec{S}_1 \cdot \vec{v}_1 \hat{n} \cdot \vec{v}_2 \vec{v}_2 \cdot \vec{v}_2 \hat{n} \cdot \vec{v}_1 - \frac{2}{3} \hat{n} \times \vec{S}_1 \cdot \vec{v}_1 (\vec{v}_1 \cdot \vec{v}_2)^2 + \frac{4}{3} \hat{n} \times \vec{S}_1 \cdot \vec{v}_1 (\hat{n} \cdot \vec{v}_2)^2 \vec{v}_1 \cdot \vec{v}_1 - \\
& \frac{2}{3} \vec{S}_1 \times \vec{v}_1 \cdot \vec{v}_2 \hat{n} \cdot \vec{v}_2 \vec{v}_1 \cdot \vec{v}_1 - \frac{1}{2} \hat{n} \times \vec{S}_1 \cdot \vec{v}_1 \vec{v}_1 \cdot \vec{v}_1 \vec{v}_1 \cdot \vec{v}_2 - \frac{1}{3} \hat{n} \times \vec{S}_1 \cdot \vec{v}_1 \vec{v}_1 \cdot \vec{v}_1 \vec{v}_2 \cdot \vec{v}_2 + \frac{3}{4} \hat{n} \times \vec{S}_1 \cdot \vec{v}_1 \vec{v}_1 \cdot \vec{v}_2 \vec{v}_2 \cdot \vec{v}_2 \Big) \\
& m_1 m_2 G^2 + m_1 m_2 \left( -\frac{4}{3} \log \left( \frac{r}{R_\theta} \right) \frac{1}{\vec{S}_1 \times \vec{a}_1 \cdot \vec{a}_2} + \frac{11}{9} \frac{1}{\vec{S}_1 \times \vec{a}_1 \cdot \vec{a}_2} + \frac{11}{18} \frac{2}{\vec{S}_1 \times \vec{v}_1 \cdot \vec{a}_2} + \frac{11}{18} \frac{1}{\vec{S}_1 \times \vec{a}_1 \cdot \vec{a}_2} - \right. \\
& \frac{4}{3} \hat{n} \times \vec{S}_1 \cdot \vec{a}_1 \hat{n} \cdot \vec{a}_2 - \frac{2}{3} \hat{n} \times \vec{S}_1 \cdot \vec{v}_1 \hat{n} \cdot \vec{a}_2 - \frac{2}{3} \hat{n} \times \vec{S}_1 \cdot \vec{a}_1 \hat{n} \cdot \vec{a}_2 - \frac{2}{3} \vec{S}_1 \times \vec{v}_1 \cdot \vec{a}_2 \log \left( \frac{r}{R_\theta} \right) - \\
& \left. \frac{2}{3} \vec{S}_1 \times \vec{a}_1 \cdot \vec{a}_2 \log \left( \frac{r}{R_\theta} \right) + \frac{\frac{2}{3} \vec{S}_1 \times \vec{a}_1 \cdot \vec{a}_2 + \frac{1}{3} \vec{S}_1 \times \vec{v}_1 \cdot \vec{a}_2 + \frac{1}{3} \vec{S}_1 \times \vec{a}_1 \cdot \vec{a}_2}{\epsilon_d} \right) G^2 \Big\}
\end{aligned}$$

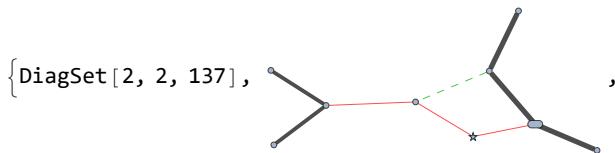

$$\begin{aligned}
& \frac{1}{r} \left( \frac{4}{3} \hat{n} \times \vec{S}_1 \cdot \vec{v}_1 (\hat{n} \cdot \vec{a}_1)^2 - \frac{2}{3} \vec{S}_1 \times \vec{v}_1 \cdot \vec{v}_2 \hat{n} \cdot \vec{a}_1 - \frac{2}{3} \vec{S}_1 \times \vec{a}_1 \cdot \vec{v}_2 \hat{n} \cdot \vec{a}_1 + 2 \vec{S}_1 \times \vec{v}_1 \cdot \vec{a}_1 \hat{n} \cdot \vec{a}_1 + \right. \\
& \frac{8}{3} \hat{n} \times \vec{S}_1 \cdot \vec{v}_1 \hat{n} \cdot \vec{v}_1 \hat{n} \cdot \vec{a}_1 + \frac{8}{3} \hat{n} \times \vec{S}_1 \cdot \vec{a}_1 \hat{n} \cdot \vec{v}_1 \hat{n} \cdot \vec{a}_1 + \frac{4}{3} \hat{n} \times \vec{S}_1 \cdot \vec{v}_1 \hat{n} \cdot \vec{v}_2 \hat{n} \cdot \vec{a}_1 + \frac{4}{3} \hat{n} \times \vec{S}_1 \cdot \vec{a}_1 \hat{n} \cdot \vec{v}_2 \hat{n} \cdot \vec{a}_1 + \\
& \frac{8}{3} \hat{n} \times \vec{S}_1 \cdot \vec{a}_1 (\hat{n} \cdot \vec{v}_1)^2 + \frac{4}{3} \hat{n} \times \vec{S}_1 \cdot \vec{v}_1 (\hat{n} \cdot \vec{v}_1)^2 + \frac{4}{3} \hat{n} \times \vec{S}_1 \cdot \vec{a}_1 (\hat{n} \cdot \vec{v}_1)^2 + \frac{8}{3} \vec{S}_1 \times \vec{v}_1 \cdot \vec{a}_1 \hat{n} \cdot \vec{a}_2 + \\
& \frac{8}{3} \vec{S}_1 \times \vec{a}_1 \cdot \vec{v}_2 \hat{n} \cdot \vec{v}_1 - \frac{8}{3} \vec{S}_1 \times \vec{v}_1 \cdot \vec{a}_1 \hat{n} \cdot \vec{v}_1 - \frac{2}{3} \vec{S}_1 \times \vec{v}_1 \cdot \vec{a}_2 \hat{n} \cdot \vec{v}_1 + \frac{4}{3} \vec{S}_1 \times \vec{v}_1 \cdot \vec{v}_2 \hat{n} \cdot \vec{v}_1 + \frac{4}{3} \vec{S}_1 \times \vec{a}_1 \cdot \vec{v}_2 \hat{n} \cdot \vec{v}_1 - \\
& \frac{2}{3} \vec{S}_1 \times \vec{a}_1 \cdot \vec{a}_2 \hat{n} \cdot \vec{v}_1 - \frac{2}{3} \vec{S}_1 \times \vec{v}_1 \cdot \vec{a}_1 \hat{n} \cdot \vec{v}_1 + \frac{4}{3} \hat{n} \times \vec{S}_1 \cdot \vec{v}_1 \hat{n} \cdot \vec{a}_2 \hat{n} \cdot \vec{v}_1 + \frac{4}{3} \hat{n} \times \vec{S}_1 \cdot \vec{a}_1 \hat{n} \cdot \vec{a}_2 \hat{n} \cdot \vec{v}_1 - \\
& \frac{16}{3} \vec{S}_1 \times \vec{v}_1 \cdot \vec{a}_1 \hat{n} \cdot \vec{v}_2 - \frac{4}{3} \vec{S}_1 \times \vec{v}_1 \cdot \vec{a}_1 \hat{n} \cdot \vec{v}_2 - \frac{16}{3} \hat{n} \times \vec{S}_1 \cdot \vec{a}_1 \hat{n} \cdot \vec{v}_1 \hat{n} \cdot \vec{v}_2 - \frac{8}{3} \hat{n} \times \vec{S}_1 \cdot \vec{v}_1 \hat{n} \cdot \vec{v}_1 \hat{n} \cdot \vec{v}_2 - \\
& \frac{8}{3} \hat{n} \times \vec{S}_1 \cdot \vec{a}_1 \hat{n} \cdot \vec{v}_1 \hat{n} \cdot \vec{v}_2 - \frac{2}{3} \hat{n} \times \vec{S}_1 \cdot \vec{v}_1 \vec{a}_1 \cdot \vec{a}_1 - \frac{2}{3} \hat{n} \times \vec{S}_1 \cdot \vec{v}_1 \vec{a}_1 \cdot \vec{v}_2 - \frac{2}{3} \hat{n} \times \vec{S}_1 \cdot \vec{a}_1 \vec{a}_1 \cdot \vec{v}_2 - \frac{4}{3} \hat{n} \times \vec{S}_1 \cdot \vec{v}_1 \vec{v}_1 \cdot \vec{a}_1 - \\
& \frac{4}{3} \hat{n} \times \vec{S}_1 \cdot \vec{a}_1 \vec{v}_1 \cdot \vec{a}_1 - \frac{2}{3} \hat{n} \times \vec{S}_1 \cdot \vec{v}_1 \vec{v}_1 \cdot \vec{a}_2 - \frac{2}{3} \hat{n} \times \vec{S}_1 \cdot \vec{a}_1 \vec{v}_1 \cdot \vec{a}_2 - \frac{4}{3} \hat{n} \times \vec{S}_1 \cdot \vec{a}_1 \vec{v}_1 \cdot \vec{v}_1 - \frac{2}{3} \hat{n} \times \vec{S}_1 \cdot \vec{v}_1 \vec{v}_1 \cdot \vec{v}_1 - \\
& \left. \frac{2}{3} \hat{n} \times \vec{S}_1 \cdot \vec{a}_1 \vec{v}_1 \cdot \vec{v}_1 + \frac{8}{3} \hat{n} \times \vec{S}_1 \cdot \vec{a}_1 \vec{v}_1 \cdot \vec{v}_2 + \frac{4}{3} \hat{n} \times \vec{S}_1 \cdot \vec{v}_1 \vec{v}_1 \cdot \vec{v}_2 + \frac{4}{3} \hat{n} \times \vec{S}_1 \cdot \vec{a}_1 \vec{v}_1 \cdot \vec{v}_2 \right) m_1 m_2 G^2 + \frac{1}{r^2} \\
& \left( -\frac{8}{3} \hat{n} \times \vec{S}_1 \cdot \vec{v}_1 (\hat{n} \cdot \vec{v}_1)^3 - \frac{8}{3} \hat{n} \times \vec{S}_1 \cdot \vec{a}_1 (\hat{n} \cdot \vec{v}_1)^3 - \frac{7}{3} \vec{S}_1 \times \vec{v}_1 \cdot \vec{v}_2 (\hat{n} \cdot \vec{v}_1)^2 - \frac{7}{3} \vec{S}_1 \times \vec{a}_1 \cdot \vec{v}_2 (\hat{n} \cdot \vec{v}_1)^2 - \right. \\
& \frac{5}{3} \vec{S}_1 \times \vec{v}_1 \cdot \vec{a}_1 (\hat{n} \cdot \vec{v}_1)^2 + \vec{S}_1 \times \vec{v}_1 \cdot \vec{a}_2 (\hat{n} \cdot \vec{v}_1)^2 - \frac{16}{3} \hat{n} \times \vec{S}_1 \cdot \vec{v}_1 \hat{n} \cdot \vec{a}_1 (\hat{n} \cdot \vec{v}_1)^2 - 4 \hat{n} \times \vec{S}_1 \cdot \vec{v}_1 \hat{n} \cdot \vec{a}_2 (\hat{n} \cdot \vec{v}_1)^2 + \\
& \frac{28}{3} \hat{n} \times \vec{S}_1 \cdot \vec{v}_1 \hat{n} \cdot \vec{v}_2 (\hat{n} \cdot \vec{v}_1)^2 + \frac{28}{3} \hat{n} \times \vec{S}_1 \cdot \vec{a}_1 \hat{n} \cdot \vec{v}_2 (\hat{n} \cdot \vec{v}_1)^2 + \frac{16}{3} \hat{n} \times \vec{S}_1 \cdot \vec{v}_1 (\hat{n} \cdot \vec{v}_2)^2 \hat{n} \cdot \vec{v}_1 + \\
& \frac{16}{3} \hat{n} \times \vec{S}_1 \cdot \vec{a}_1 (\hat{n} \cdot \vec{v}_2)^2 \hat{n} \cdot \vec{v}_1 - \frac{1}{3} \vec{S}_1 \times \vec{v}_1 \cdot \vec{v}_2 \hat{n} \cdot \vec{a}_1 \hat{n} \cdot \vec{v}_1 - \frac{8}{3} \vec{S}_1 \times \vec{v}_1 \cdot \vec{v}_2 \hat{n} \cdot \vec{v}_2 \hat{n} \cdot \vec{v}_1 - \frac{8}{3} \vec{S}_1 \times \vec{a}_1 \cdot \vec{v}_2 \hat{n} \cdot \vec{v}_2 \hat{n} \cdot \vec{v}_1 + \\
& \left. \frac{22}{3} \vec{S}_1 \times \vec{v}_1 \cdot \vec{a}_1 \hat{n} \cdot \vec{v}_2 \hat{n} \cdot \vec{v}_1 + \frac{4}{3} \hat{n} \times \vec{S}_1 \cdot \vec{v}_1 \hat{n} \cdot \vec{a}_1 \hat{n} \cdot \vec{v}_2 \hat{n} \cdot \vec{v}_1 - \frac{1}{3} \hat{n} \times \vec{S}_1 \cdot \vec{v}_1 \vec{a}_1 \cdot \vec{v}_2 \hat{n} \cdot \vec{v}_1 + \right.
\end{aligned}$$

$$\begin{aligned}
& \frac{5}{3} \hat{n} \times \vec{S}_1 \cdot \vec{v}_1 \vec{v}_1 \cdot \vec{a}_1 \hat{n} \cdot \vec{v}_1 + 2 \hat{n} \times \vec{S}_1 \cdot \vec{v}_1 \vec{v}_1 \cdot \vec{a}_2 \hat{n} \cdot \vec{v}_1 - \frac{14}{3} \hat{n} \times \vec{S}_1 \cdot \vec{v}_1 \vec{v}_1 \cdot \vec{v}_2 \hat{n} \cdot \vec{v}_1 - \frac{14}{3} \hat{n} \times \vec{S}_1 \cdot \vec{a}_1 \vec{v}_1 \cdot \vec{v}_2 \hat{n} \cdot \vec{v}_1 - \\
& \frac{4}{3} \hat{n} \times \vec{S}_1 \cdot \vec{v}_1 \vec{v}_2 \cdot \vec{v}_2 \hat{n} \cdot \vec{v}_1 - \frac{4}{3} \hat{n} \times \vec{S}_1 \cdot \vec{a}_1 \vec{v}_2 \cdot \vec{v}_2 \hat{n} \cdot \vec{v}_1 + \frac{16}{3} \vec{S}_1 \times \vec{v}_1 \cdot \vec{a}_1 (\hat{n} \cdot \vec{v}_2)^2 - \frac{1}{3} \vec{S}_1 \times \vec{v}_1 \cdot \vec{v}_2 \vec{v}_1 \cdot \vec{a}_1 + \\
& \frac{2}{3} \hat{n} \times \vec{S}_1 \cdot \vec{v}_1 \hat{n} \cdot \vec{v}_2 \vec{v}_1 \cdot \vec{a}_1 + \frac{5}{3} \vec{S}_1 \times \vec{v}_1 \cdot \vec{v}_2 \vec{v}_1 \cdot \vec{v}_1 + \frac{5}{3} \vec{S}_1 \times \vec{a}_1 \cdot \vec{v}_2 \vec{v}_1 \cdot \vec{v}_1 - \frac{2}{3} \vec{S}_1 \times \vec{v}_1 \cdot \vec{a}_1 \vec{v}_1 \cdot \vec{v}_1 - \\
& \vec{S}_1 \times \vec{v}_1 \cdot \vec{a}_2 \vec{v}_1 \cdot \vec{v}_1 + \frac{7}{3} \hat{n} \times \vec{S}_1 \cdot \vec{v}_1 \hat{n} \cdot \vec{a}_1 \vec{v}_1 \cdot \vec{v}_1 + 2 \hat{n} \times \vec{S}_1 \cdot \vec{v}_1 \hat{n} \cdot \vec{a}_2 \vec{v}_1 \cdot \vec{v}_1 - \frac{10}{3} \hat{n} \times \vec{S}_1 \cdot \vec{v}_1 \hat{n} \cdot \vec{v}_2 \vec{v}_1 \cdot \vec{v}_1 - \\
& \frac{10}{3} \hat{n} \times \vec{S}_1 \cdot \vec{a}_1 \hat{n} \cdot \vec{v}_2 \vec{v}_1 \cdot \vec{v}_1 + \frac{4}{3} \vec{S}_1 \times \vec{v}_1 \cdot \vec{v}_2 \vec{v}_1 \cdot \vec{v}_2 + \frac{4}{3} \vec{S}_1 \times \vec{a}_1 \cdot \vec{v}_2 \vec{v}_1 \cdot \vec{v}_2 - \frac{11}{3} \vec{S}_1 \times \vec{v}_1 \cdot \vec{a}_1 \vec{v}_1 \cdot \vec{v}_2 - \\
& \frac{1}{3} \hat{n} \times \vec{S}_1 \cdot \vec{v}_1 \hat{n} \cdot \vec{a}_1 \vec{v}_1 \cdot \vec{v}_2 - \frac{8}{3} \hat{n} \times \vec{S}_1 \cdot \vec{v}_1 \hat{n} \cdot \vec{v}_2 \vec{v}_1 \cdot \vec{v}_2 - \frac{8}{3} \hat{n} \times \vec{S}_1 \cdot \vec{a}_1 \hat{n} \cdot \vec{v}_2 \vec{v}_1 \cdot \vec{v}_2 - \frac{8}{3} \vec{S}_1 \times \vec{v}_1 \cdot \vec{a}_1 \vec{v}_2 \cdot \vec{v}_2 \Big) m_1 m_2 G^2 + \frac{1}{r^3} \\
& \left( 4 \hat{n} \times \vec{S}_1 \cdot \vec{v}_1 (\hat{n} \cdot \vec{v}_1)^4 + \frac{10}{3} \vec{S}_1 \times \vec{v}_1 \cdot \vec{v}_2 (\hat{n} \cdot \vec{v}_1)^3 - 20 \hat{n} \times \vec{S}_1 \cdot \vec{v}_1 \hat{n} \cdot \vec{v}_2 (\hat{n} \cdot \vec{v}_1)^3 - 24 \hat{n} \times \vec{S}_1 \cdot \vec{v}_1 (\hat{n} \cdot \vec{v}_2)^2 (\hat{n} \cdot \vec{v}_1)^2 + \right. \\
& 8 \vec{S}_1 \times \vec{v}_1 \cdot \vec{v}_2 \hat{n} \cdot \vec{v}_2 (\hat{n} \cdot \vec{v}_1)^2 - 2 \hat{n} \times \vec{S}_1 \cdot \vec{v}_1 \vec{v}_1 \cdot \vec{v}_1 (\hat{n} \cdot \vec{v}_1)^2 + 10 \hat{n} \times \vec{S}_1 \cdot \vec{v}_1 \vec{v}_1 \cdot \vec{v}_2 (\hat{n} \cdot \vec{v}_1)^2 + \\
& 4 \hat{n} \times \vec{S}_1 \cdot \vec{v}_1 \vec{v}_2 \cdot \vec{v}_2 (\hat{n} \cdot \vec{v}_1)^2 - 4 \vec{S}_1 \times \vec{v}_1 \cdot \vec{v}_2 \vec{v}_1 \cdot \vec{v}_1 \hat{n} \cdot \vec{v}_1 + 16 \hat{n} \times \vec{S}_1 \cdot \vec{v}_1 \hat{n} \cdot \vec{v}_2 \vec{v}_1 \cdot \vec{v}_1 \hat{n} \cdot \vec{v}_1 - \\
& 4 \vec{S}_1 \times \vec{v}_1 \cdot \vec{v}_2 \vec{v}_1 \cdot \vec{v}_2 \hat{n} \cdot \vec{v}_1 + 16 \hat{n} \times \vec{S}_1 \cdot \vec{v}_1 \hat{n} \cdot \vec{v}_2 \vec{v}_1 \cdot \vec{v}_2 \hat{n} \cdot \vec{v}_1 - 2 \hat{n} \times \vec{S}_1 \cdot \vec{v}_1 (\vec{v}_1 \cdot \vec{v}_2)^2 + 8 \hat{n} \times \vec{S}_1 \cdot \vec{v}_1 (\hat{n} \cdot \vec{v}_2)^2 \vec{v}_1 \cdot \vec{v}_1 - \\
& \left. 4 \vec{S}_1 \times \vec{v}_1 \cdot \vec{v}_2 \hat{n} \cdot \vec{v}_2 \vec{v}_1 \cdot \vec{v}_1 - 4 \hat{n} \times \vec{S}_1 \cdot \vec{v}_1 \vec{v}_1 \cdot \vec{v}_1 \vec{v}_1 \cdot \vec{v}_2 - 2 \hat{n} \times \vec{S}_1 \cdot \vec{v}_1 \vec{v}_1 \cdot \vec{v}_1 \vec{v}_2 \cdot \vec{v}_2 \right) m_1 m_2 G^2 + \\
& m_1 m_2 \left( -\frac{4}{3} \log\left(\frac{r}{R_0}\right) \vec{S}_1 \times \vec{v}_1 \cdot \vec{a}_1 + \frac{2}{9} \vec{S}_1 \times \vec{v}_1 \cdot \vec{a}_1 - \frac{2}{9} \vec{S}_1 \times \vec{a}_1 \cdot \vec{a}_1 - \frac{8}{3} \hat{n} \times \vec{S}_1 \cdot \vec{a}_1 \hat{n} \cdot \vec{a}_1 - \frac{4}{3} \hat{n} \times \vec{S}_1 \cdot \vec{v}_1 \hat{n} \cdot \vec{a}_1 - \right. \\
& \left. \frac{4}{3} \hat{n} \times \vec{S}_1 \cdot \vec{a}_1 \hat{n} \cdot \vec{a}_1 + \frac{4}{3} \vec{S}_1 \times \vec{a}_1 \cdot \vec{a}_1 \log\left(\frac{r}{R_0}\right) + \frac{\frac{2}{3} \vec{S}_1 \times \vec{v}_1 \cdot \vec{a}_1 - \frac{2}{3} \vec{S}_1 \times \vec{a}_1 \cdot \vec{a}_1}{\epsilon_d} \right) G^2 \Big\}
\end{aligned}$$

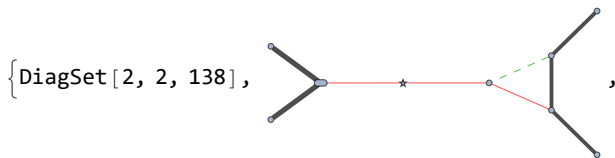

$$\begin{aligned}
& \frac{1}{r} G^2 \left( \frac{8}{3} \hat{n} \times \vec{a}_1 \cdot \vec{S}_1 (\hat{n} \cdot \vec{v}_2)^2 - \frac{8}{3} \hat{n} \times \vec{S}_1 \cdot \vec{v}_1 (\hat{n} \cdot \vec{v}_2)^2 + \frac{16}{3} \hat{n} \times \vec{a}_1 \cdot \vec{S}_1 (\hat{n} \cdot \vec{v}_2)^2 - \frac{8}{3} \vec{a}_1 \times \vec{S}_1 \cdot \vec{v}_2 \hat{n} \cdot \vec{v}_2 + \frac{8}{3} \vec{S}_1 \times \vec{v}_1 \cdot \vec{v}_2 \hat{n} \cdot \vec{v}_2 - \right. \\
& \frac{16}{3} \vec{a}_1 \times \vec{S}_1 \cdot \vec{v}_2 \hat{n} \cdot \vec{v}_2 - \frac{8}{3} \vec{a}_1 \times \vec{a}_2 \cdot \vec{S}_1 \hat{n} \cdot \vec{v}_2 - \frac{8}{3} \vec{a}_2 \times \vec{S}_1 \cdot \vec{v}_1 \hat{n} \cdot \vec{v}_2 + \frac{16}{3} \hat{n} \times \vec{S}_1 \cdot \vec{v}_1 \hat{n} \cdot \vec{a}_2 \hat{n} \cdot \vec{v}_2 - \\
& \frac{16}{3} \hat{n} \times \vec{a}_1 \cdot \vec{S}_1 \hat{n} \cdot \vec{a}_2 \hat{n} \cdot \vec{v}_2 - \frac{4}{3} \vec{a}_2 \times \vec{S}_1 \cdot \vec{v}_1 \hat{n} \cdot \vec{a}_1 - \frac{8}{3} \vec{S}_1 \times \vec{v}_1 \cdot \vec{v}_2 \hat{n} \cdot \vec{a}_2 + \frac{4}{3} \vec{a}_1 \times \vec{S}_1 \cdot \vec{v}_1 \hat{n} \cdot \vec{a}_2 + \frac{8}{3} \vec{a}_1 \times \vec{S}_1 \cdot \vec{v}_2 \hat{n} \cdot \vec{a}_2 + \\
& \frac{8}{3} \hat{n} \times \vec{S}_1 \cdot \vec{v}_1 \hat{n} \cdot \vec{a}_1 \hat{n} \cdot \vec{a}_2 - \frac{8}{3} \vec{a}_1 \times \vec{a}_2 \cdot \vec{S}_1 \hat{n} \cdot \vec{v}_1 - \frac{8}{3} \vec{a}_2 \times \vec{S}_1 \cdot \vec{v}_1 \hat{n} \cdot \vec{v}_1 + \frac{16}{3} \hat{n} \times \vec{S}_1 \cdot \vec{v}_1 \hat{n} \cdot \vec{a}_2 \hat{n} \cdot \vec{v}_1 - \\
& \frac{16}{3} \hat{n} \times \vec{a}_1 \cdot \vec{S}_1 \hat{n} \cdot \vec{a}_2 \hat{n} \cdot \vec{v}_1 - \frac{4}{3} \hat{n} \times \vec{S}_1 \cdot \vec{v}_1 \vec{a}_1 \cdot \vec{a}_2 - \frac{8}{3} \hat{n} \times \vec{S}_1 \cdot \vec{v}_1 \vec{a}_2 \cdot \vec{v}_1 + \frac{8}{3} \hat{n} \times \vec{a}_1 \cdot \vec{S}_1 \vec{a}_2 \cdot \vec{v}_1 - \\
& \frac{8}{3} \hat{n} \times \vec{S}_1 \cdot \vec{v}_1 \vec{a}_2 \cdot \vec{v}_2 + \frac{8}{3} \hat{n} \times \vec{a}_1 \cdot \vec{S}_1 \vec{a}_2 \cdot \vec{v}_2 - \frac{4}{3} \hat{n} \times \vec{a}_1 \cdot \vec{S}_1 \vec{v}_2 \cdot \vec{v}_2 + \frac{4}{3} \hat{n} \times \vec{S}_1 \cdot \vec{v}_1 \vec{v}_2 \cdot \vec{v}_2 - \frac{8}{3} \hat{n} \times \vec{a}_1 \cdot \vec{S}_1 \vec{v}_2 \cdot \vec{v}_2 \Big) m_2^2 + \\
& \frac{1}{r^2} G^2 \left( \frac{32}{3} \hat{n} \times \vec{S}_1 \cdot \vec{v}_1 (\hat{n} \cdot \vec{v}_2)^3 - \frac{32}{3} \hat{n} \times \vec{a}_1 \cdot \vec{S}_1 (\hat{n} \cdot \vec{v}_2)^3 - 8 \vec{S}_1 \times \vec{v}_1 \cdot \vec{v}_2 (\hat{n} \cdot \vec{v}_2)^2 + \frac{8}{3} \vec{a}_1 \times \vec{S}_1 \cdot \vec{v}_1 (\hat{n} \cdot \vec{v}_2)^2 + \right. \\
& 8 \vec{a}_1 \times \vec{S}_1 \cdot \vec{v}_2 (\hat{n} \cdot \vec{v}_2)^2 + \frac{32}{3} \hat{n} \times \vec{S}_1 \cdot \vec{v}_1 \hat{n} \cdot \vec{a}_1 (\hat{n} \cdot \vec{v}_2)^2 + \frac{64}{3} \hat{n} \times \vec{S}_1 \cdot \vec{v}_1 \hat{n} \cdot \vec{v}_1 (\hat{n} \cdot \vec{v}_2)^2 - \\
& \left. \frac{64}{3} \hat{n} \times \vec{a}_1 \cdot \vec{S}_1 \hat{n} \cdot \vec{v}_1 (\hat{n} \cdot \vec{v}_2)^2 - \frac{16}{3} \vec{S}_1 \times \vec{v}_1 \cdot \vec{v}_2 \hat{n} \cdot \vec{a}_1 \hat{n} \cdot \vec{v}_2 - \frac{32}{3} \vec{S}_1 \times \vec{v}_1 \cdot \vec{v}_2 \hat{n} \cdot \vec{v}_1 \hat{n} \cdot \vec{v}_2 + \frac{32}{3} \vec{a}_1 \times \vec{S}_1 \cdot \vec{v}_2 \hat{n} \cdot \vec{v}_1 \hat{n} \cdot \vec{v}_2 + \right.
\end{aligned}$$

$$\begin{aligned}
& \frac{16}{3} \vec{a}_2 \times \vec{S}_1 \cdot \vec{v}_1 \hat{n} \cdot \vec{v}_1 \hat{n} \cdot \vec{v}_2 - \frac{64}{3} \hat{n} \times \vec{S}_1 \cdot \vec{v}_1 \hat{n} \cdot \vec{a}_2 \hat{n} \cdot \vec{v}_1 \hat{n} \cdot \vec{v}_2 - \frac{16}{3} \hat{n} \times \vec{S}_1 \cdot \vec{v}_1 \vec{a}_1 \cdot \vec{v}_2 \hat{n} \cdot \vec{v}_2 + \\
& \frac{16}{3} \hat{n} \times \vec{S}_1 \cdot \vec{v}_1 \vec{a}_2 \cdot \vec{v}_1 \hat{n} \cdot \vec{v}_2 - \frac{32}{3} \hat{n} \times \vec{S}_1 \cdot \vec{v}_1 \vec{v}_1 \cdot \vec{v}_2 \hat{n} \cdot \vec{v}_2 + \frac{32}{3} \hat{n} \times \vec{a}_1 \cdot \vec{S}_1 \vec{v}_1 \cdot \vec{v}_2 \hat{n} \cdot \vec{v}_2 - 8 \hat{n} \times \vec{S}_1 \cdot \vec{v}_1 \vec{v}_2 \cdot \vec{v}_2 \hat{n} \cdot \vec{v}_2 + \\
& 8 \hat{n} \times \vec{a}_1 \cdot \vec{S}_1 \vec{v}_2 \cdot \vec{v}_2 \hat{n} \cdot \vec{v}_2 + \frac{8}{3} \vec{a}_2 \times \vec{S}_1 \cdot \vec{v}_1 (\hat{n} \cdot \vec{v}_1)^2 - \frac{32}{3} \hat{n} \times \vec{S}_1 \cdot \vec{v}_1 \hat{n} \cdot \vec{a}_2 (\hat{n} \cdot \vec{v}_1)^2 + \frac{16}{3} \vec{S}_1 \times \vec{v}_1 \cdot \vec{v}_2 \hat{n} \cdot \vec{a}_2 \hat{n} \cdot \vec{v}_1 + \\
& \frac{8}{3} \vec{S}_1 \times \vec{v}_1 \cdot \vec{v}_2 \vec{a}_1 \cdot \vec{v}_2 - \frac{8}{3} \vec{S}_1 \times \vec{v}_1 \cdot \vec{v}_2 \vec{a}_2 \cdot \vec{v}_1 + \frac{16}{3} \hat{n} \times \vec{S}_1 \cdot \vec{v}_1 \hat{n} \cdot \vec{v}_1 \vec{a}_2 \cdot \vec{v}_1 + \frac{16}{3} \hat{n} \times \vec{S}_1 \cdot \vec{v}_1 \hat{n} \cdot \vec{v}_1 \vec{a}_2 \cdot \vec{v}_2 - \\
& \frac{4}{3} \vec{a}_2 \times \vec{S}_1 \cdot \vec{v}_1 \vec{v}_1 \cdot \vec{v}_1 + \frac{8}{3} \hat{n} \times \vec{S}_1 \cdot \vec{v}_1 \hat{n} \cdot \vec{a}_2 \vec{v}_1 \cdot \vec{v}_1 + \frac{16}{3} \vec{S}_1 \times \vec{v}_1 \cdot \vec{v}_2 \vec{v}_1 \cdot \vec{v}_2 - \frac{16}{3} \vec{a}_1 \times \vec{S}_1 \cdot \vec{v}_2 \vec{v}_1 \cdot \vec{v}_2 - \\
& \frac{8}{3} \vec{a}_2 \times \vec{S}_1 \cdot \vec{v}_1 \vec{v}_1 \cdot \vec{v}_2 + \frac{16}{3} \hat{n} \times \vec{S}_1 \cdot \vec{v}_1 \hat{n} \cdot \vec{a}_2 \vec{v}_1 \cdot \vec{v}_2 + 4 \vec{S}_1 \times \vec{v}_1 \cdot \vec{v}_2 \vec{v}_2 \cdot \vec{v}_2 - \frac{4}{3} \vec{a}_1 \times \vec{S}_1 \cdot \vec{v}_1 \vec{v}_2 \cdot \vec{v}_2 - \\
& 4 \vec{a}_1 \times \vec{S}_1 \cdot \vec{v}_2 \vec{v}_2 \cdot \vec{v}_2 - \frac{8}{3} \hat{n} \times \vec{S}_1 \cdot \vec{v}_1 \hat{n} \cdot \vec{a}_1 \vec{v}_2 \cdot \vec{v}_2 - \frac{16}{3} \hat{n} \times \vec{S}_1 \cdot \vec{v}_1 \hat{n} \cdot \vec{v}_1 \vec{v}_2 \cdot \vec{v}_2 + \frac{16}{3} \hat{n} \times \vec{a}_1 \cdot \vec{S}_1 \hat{n} \cdot \vec{v}_1 \vec{v}_2 \cdot \vec{v}_2 \Big) m_2^2 + \\
& \frac{1}{r^3} G^2 \left( -64 \hat{n} \times \vec{S}_1 \cdot \vec{v}_1 \hat{n} \cdot \vec{v}_1 (\hat{n} \cdot \vec{v}_2)^3 - 64 \hat{n} \times \vec{S}_1 \cdot \vec{v}_1 (\hat{n} \cdot \vec{v}_1)^2 (\hat{n} \cdot \vec{v}_2)^2 + 32 \vec{S}_1 \times \vec{v}_1 \cdot \vec{v}_2 \hat{n} \cdot \vec{v}_1 (\hat{n} \cdot \vec{v}_2)^2 + \right. \\
& \frac{32}{3} \hat{n} \times \vec{S}_1 \cdot \vec{v}_1 \vec{v}_1 \cdot \vec{v}_1 (\hat{n} \cdot \vec{v}_2)^2 + 32 \hat{n} \times \vec{S}_1 \cdot \vec{v}_1 \vec{v}_1 \cdot \vec{v}_2 (\hat{n} \cdot \vec{v}_2)^2 + \frac{64}{3} \vec{S}_1 \times \vec{v}_1 \cdot \vec{v}_2 (\hat{n} \cdot \vec{v}_1)^2 \hat{n} \cdot \vec{v}_2 - \\
& \frac{16}{3} \vec{S}_1 \times \vec{v}_1 \cdot \vec{v}_2 \vec{v}_1 \cdot \vec{v}_1 \hat{n} \cdot \vec{v}_2 - 16 \vec{S}_1 \times \vec{v}_1 \cdot \vec{v}_2 \vec{v}_1 \cdot \vec{v}_2 \hat{n} \cdot \vec{v}_2 + \frac{128}{3} \hat{n} \times \vec{S}_1 \cdot \vec{v}_1 \hat{n} \cdot \vec{v}_1 \vec{v}_1 \cdot \vec{v}_2 \hat{n} \cdot \vec{v}_2 + \\
& 32 \hat{n} \times \vec{S}_1 \cdot \vec{v}_1 \hat{n} \cdot \vec{v}_1 \vec{v}_2 \cdot \vec{v}_2 \hat{n} \cdot \vec{v}_2 - \frac{16}{3} \hat{n} \times \vec{S}_1 \cdot \vec{v}_1 (\vec{v}_1 \cdot \vec{v}_2)^2 - \frac{32}{3} \vec{S}_1 \times \vec{v}_1 \cdot \vec{v}_2 \hat{n} \cdot \vec{v}_1 \vec{v}_1 \cdot \vec{v}_2 + \\
& \left. \frac{32}{3} \hat{n} \times \vec{S}_1 \cdot \vec{v}_1 (\hat{n} \cdot \vec{v}_1)^2 \vec{v}_2 \cdot \vec{v}_2 - 8 \vec{S}_1 \times \vec{v}_1 \cdot \vec{v}_2 \hat{n} \cdot \vec{v}_1 \vec{v}_2 \cdot \vec{v}_2 - \frac{8}{3} \hat{n} \times \vec{S}_1 \cdot \vec{v}_1 \vec{v}_1 \cdot \vec{v}_1 \vec{v}_2 \cdot \vec{v}_2 - 8 \hat{n} \times \vec{S}_1 \cdot \vec{v}_1 \vec{v}_1 \cdot \vec{v}_2 \vec{v}_2 \cdot \vec{v}_2 \right) \\
& m_2^2 + G^2 \left( -\frac{4}{3} \log\left(\frac{r}{R_\theta}\right) \frac{1}{\vec{a}_1 \times \vec{a}_2 \cdot \vec{S}_1} + \frac{8}{9} \frac{1}{\vec{a}_1 \times \vec{a}_2 \cdot \vec{S}_1} + \frac{16}{9} \vec{a}_1 \times \vec{a}_2 \cdot \frac{1}{\vec{S}_1} + \frac{8}{9} \vec{a}_2 \times \vec{S}_1 \cdot \frac{1}{\vec{v}_1} + \right. \\
& \frac{4}{3} \hat{n} \times \frac{1}{\vec{a}_1} \cdot \vec{S}_1 \hat{n} \cdot \vec{a}_2 - \frac{4}{3} \hat{n} \times \vec{S}_1 \cdot \vec{v}_1 \hat{n} \cdot \vec{a}_2 + \frac{8}{3} \hat{n} \times \vec{a}_1 \cdot \vec{S}_1 \hat{n} \cdot \vec{a}_2 - \frac{8}{3} \vec{a}_1 \times \vec{a}_2 \cdot \vec{S}_1 \log\left(\frac{r}{R_\theta}\right) - \\
& \left. \frac{4}{3} \vec{a}_2 \times \vec{S}_1 \cdot \vec{v}_1 \log\left(\frac{r}{R_\theta}\right) + \frac{\frac{2}{3} \vec{a}_1 \times \vec{a}_2 \cdot \vec{S}_1 + \frac{4}{3} \vec{a}_1 \times \vec{a}_2 \cdot \frac{1}{\vec{S}_1} + \frac{2}{3} \vec{a}_2 \times \vec{S}_1 \cdot \frac{1}{\vec{v}_1}}{\epsilon_d} \right) m_2^2 \Big\}
\end{aligned}$$

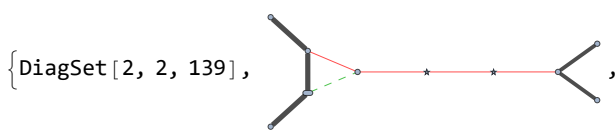

$$\begin{aligned}
& \frac{1}{r} \left( \frac{1}{3} \hat{n} \times \vec{S}_1 \cdot \vec{a}_1 (\hat{n} \cdot \vec{v}_2)^2 + \frac{1}{6} \hat{n} \times \vec{S}_1 \cdot \vec{v}_1 (\hat{n} \cdot \vec{v}_2)^2 + \frac{1}{6} \hat{n} \times \vec{S}_1 \cdot \vec{a}_1 (\hat{n} \cdot \vec{v}_2)^2 - \frac{1}{3} \vec{S}_1 \times \vec{a}_1 \cdot \vec{v}_2 \hat{n} \cdot \vec{v}_2 - \frac{1}{6} \vec{S}_1 \times \vec{v}_1 \cdot \vec{v}_2 \hat{n} \cdot \vec{v}_2 - \right. \\
& \frac{1}{6} \vec{S}_1 \times \vec{a}_1 \cdot \vec{v}_2 \hat{n} \cdot \vec{v}_2 + \frac{1}{12} \vec{S}_1 \times \vec{v}_1 \cdot \vec{a}_2 \hat{n} \cdot \vec{a}_1 - \frac{1}{12} \vec{S}_1 \times \vec{v}_1 \cdot \vec{a}_1 \hat{n} \cdot \vec{a}_2 - \frac{1}{6} \hat{n} \times \vec{S}_1 \cdot \vec{v}_1 \hat{n} \cdot \vec{a}_1 \hat{n} \cdot \vec{a}_2 + \frac{1}{6} \vec{S}_1 \times \vec{v}_1 \cdot \vec{a}_2 \hat{n} \cdot \vec{v}_1 + \\
& \frac{1}{6} \vec{S}_1 \times \vec{a}_1 \cdot \vec{a}_2 \hat{n} \cdot \vec{v}_1 - \frac{1}{3} \hat{n} \times \vec{S}_1 \cdot \vec{v}_1 \hat{n} \cdot \vec{a}_2 \hat{n} \cdot \vec{v}_1 - \frac{1}{3} \hat{n} \times \vec{S}_1 \cdot \vec{a}_1 \hat{n} \cdot \vec{a}_2 \hat{n} \cdot \vec{v}_1 + \frac{1}{12} \hat{n} \times \vec{S}_1 \cdot \vec{v}_1 \vec{a}_1 \cdot \vec{a}_2 + \\
& \left. \frac{1}{6} \hat{n} \times \vec{S}_1 \cdot \vec{v}_1 \vec{v}_1 \cdot \vec{a}_2 + \frac{1}{6} \hat{n} \times \vec{S}_1 \cdot \vec{a}_1 \vec{v}_1 \cdot \vec{a}_2 - \frac{1}{6} \hat{n} \times \vec{S}_1 \cdot \vec{a}_1 \vec{v}_2 \cdot \vec{v}_2 - \frac{1}{12} \hat{n} \times \vec{S}_1 \cdot \vec{v}_1 \vec{v}_2 \cdot \vec{v}_2 - \frac{1}{12} \hat{n} \times \vec{S}_1 \cdot \vec{a}_1 \vec{v}_2 \cdot \vec{v}_2 \right) \\
& m_1 m_2 G^2 + \frac{1}{r^2} \left( -\frac{1}{6} \vec{S}_1 \times \vec{v}_1 \cdot \vec{a}_2 (\hat{n} \cdot \vec{v}_1)^2 + \frac{2}{3} \hat{n} \times \vec{S}_1 \cdot \vec{v}_1 \hat{n} \cdot \vec{a}_2 (\hat{n} \cdot \vec{v}_1)^2 - \frac{4}{3} \hat{n} \times \vec{S}_1 \cdot \vec{v}_1 (\hat{n} \cdot \vec{v}_2)^2 \hat{n} \cdot \vec{v}_1 - \right. \\
& \frac{4}{3} \hat{n} \times \vec{S}_1 \cdot \vec{a}_1 (\hat{n} \cdot \vec{v}_2)^2 \hat{n} \cdot \vec{v}_1 + \frac{2}{3} \vec{S}_1 \times \vec{v}_1 \cdot \vec{v}_2 \hat{n} \cdot \vec{v}_2 \hat{n} \cdot \vec{v}_1 + \frac{2}{3} \vec{S}_1 \times \vec{a}_1 \cdot \vec{v}_2 \hat{n} \cdot \vec{v}_2 \hat{n} \cdot \vec{v}_1 - \frac{1}{3} \hat{n} \times \vec{S}_1 \cdot \vec{v}_1 \vec{v}_1 \cdot \vec{a}_2 \hat{n} \cdot \vec{v}_1 + \\
& \left. \frac{1}{3} \hat{n} \times \vec{S}_1 \cdot \vec{v}_1 \vec{v}_2 \cdot \vec{v}_2 \hat{n} \cdot \vec{v}_1 + \frac{1}{3} \hat{n} \times \vec{S}_1 \cdot \vec{a}_1 \vec{v}_2 \cdot \vec{v}_2 \hat{n} \cdot \vec{v}_1 - \frac{1}{6} \vec{S}_1 \times \vec{v}_1 \cdot \vec{a}_1 (\hat{n} \cdot \vec{v}_2)^2 - \frac{2}{3} \hat{n} \times \vec{S}_1 \cdot \vec{v}_1 \hat{n} \cdot \vec{a}_1 (\hat{n} \cdot \vec{v}_2)^2 + \right.
\end{aligned}$$



$$\begin{aligned} & \frac{1}{3} \vec{S}_1 \times \vec{v}_1 \cdot \vec{v}_2 \hat{n} \cdot \vec{a}_1 \hat{n} \cdot \vec{v}_2 - \frac{1}{6} \vec{S}_1 \times \vec{v}_1 \cdot \vec{v}_2 \vec{a}_1 \cdot \vec{v}_2 + \frac{1}{3} \hat{n} \times \vec{S}_1 \cdot \vec{v}_1 \hat{n} \cdot \vec{v}_2 \vec{a}_1 \cdot \vec{v}_2 + \frac{1}{12} \vec{S}_1 \times \vec{v}_1 \cdot \vec{a}_2 \vec{v}_1 \cdot \vec{v}_1 - \\ & \frac{1}{6} \hat{n} \times \vec{S}_1 \cdot \vec{v}_1 \hat{n} \cdot \vec{a}_2 \vec{v}_1 \cdot \vec{v}_1 - \frac{1}{3} \frac{1}{\vec{S}_1} \times \vec{v}_1 \cdot \vec{v}_2 \vec{v}_1 \cdot \vec{v}_2 - \frac{1}{3} \vec{S}_1 \times \vec{a}_1 \cdot \vec{v}_2 \vec{v}_1 \cdot \vec{v}_2 + \frac{2}{3} \hat{n} \times \vec{S}_1 \cdot \vec{v}_1 \hat{n} \cdot \vec{v}_2 \vec{v}_1 \cdot \vec{v}_2 + \\ & \frac{2}{3} \hat{n} \times \vec{S}_1 \cdot \vec{a}_1 \hat{n} \cdot \vec{v}_2 \vec{v}_1 \cdot \vec{v}_2 + \frac{1}{12} \vec{S}_1 \times \vec{v}_1 \cdot \vec{a}_1 \vec{v}_2 \cdot \vec{v}_2 + \frac{1}{6} \hat{n} \times \vec{S}_1 \cdot \vec{v}_1 \hat{n} \cdot \vec{a}_1 \vec{v}_2 \cdot \vec{v}_2 \Big) m_1 m_2 G^2 + \\ & \frac{1}{r^3} \left( 4 \hat{n} \times \vec{S}_1 \cdot \vec{v}_1 (\hat{n} \cdot \vec{v}_2)^2 (\hat{n} \cdot \vec{v}_1)^2 - \frac{4}{3} \vec{S}_1 \times \vec{v}_1 \cdot \vec{v}_2 \hat{n} \cdot \vec{v}_2 (\hat{n} \cdot \vec{v}_1)^2 - \frac{2}{3} \hat{n} \times \vec{S}_1 \cdot \vec{v}_1 \vec{v}_2 \cdot \vec{v}_2 (\hat{n} \cdot \vec{v}_1)^2 + \right. \\ & \frac{2}{3} \vec{S}_1 \times \vec{v}_1 \cdot \vec{v}_2 \vec{v}_1 \cdot \vec{v}_2 \hat{n} \cdot \vec{v}_1 - \frac{8}{3} \hat{n} \times \vec{S}_1 \cdot \vec{v}_1 \hat{n} \cdot \vec{v}_2 \vec{v}_1 \cdot \vec{v}_2 \hat{n} \cdot \vec{v}_1 + \frac{1}{3} \hat{n} \times \vec{S}_1 \cdot \vec{v}_1 (\vec{v}_1 \cdot \vec{v}_2)^2 - \\ & \left. \frac{2}{3} \hat{n} \times \vec{S}_1 \cdot \vec{v}_1 (\hat{n} \cdot \vec{v}_2)^2 \vec{v}_1 \cdot \vec{v}_1 + \frac{1}{3} \vec{S}_1 \times \vec{v}_1 \cdot \vec{v}_2 \hat{n} \cdot \vec{v}_2 \vec{v}_1 \cdot \vec{v}_1 + \frac{1}{6} \hat{n} \times \vec{S}_1 \cdot \vec{v}_1 \vec{v}_1 \cdot \vec{v}_1 \vec{v}_2 \cdot \vec{v}_2 \right) m_1 m_2 G^2 + \\ & m_1 m_2 \left( \frac{1}{6} \log \left( \frac{r}{R_\theta} \right) \frac{1}{\vec{S}_1} \times \vec{a}_1 \cdot \vec{a}_2 - \frac{1}{9} \vec{S}_1 \times \vec{a}_1 \cdot \vec{a}_2 - \frac{1}{18} \vec{S}_1 \times \vec{v}_1 \cdot \vec{a}_2 - \frac{1}{18} \vec{S}_1 \times \frac{1}{\vec{a}_1} \cdot \vec{a}_2 + \frac{1}{6} \hat{n} \times \vec{S}_1 \cdot \vec{a}_1 \hat{n} \cdot \vec{a}_2 + \right. \\ & \frac{1}{12} \hat{n} \times \vec{S}_1 \cdot \vec{v}_1 \hat{n} \cdot \vec{a}_2 + \frac{1}{12} \hat{n} \times \vec{S}_1 \cdot \vec{a}_1 \hat{n} \cdot \vec{a}_2 + \frac{1}{12} \vec{S}_1 \times \vec{v}_1 \cdot \vec{a}_2 \log \left( \frac{r}{R_\theta} \right) + \\ & \left. \frac{1}{12} \vec{S}_1 \times \vec{a}_1 \cdot \vec{a}_2 \log \left( \frac{r}{R_\theta} \right) + \frac{-\frac{1}{12} \vec{S}_1 \times \vec{a}_1 \cdot \vec{a}_2 - \frac{1}{24} \vec{S}_1 \times \vec{v}_1 \cdot \vec{a}_2 - \frac{1}{24} \vec{S}_1 \times \frac{1}{\vec{a}_1} \cdot \vec{a}_2}{\epsilon_d} \right) G^2 \Big\} \end{aligned}$$

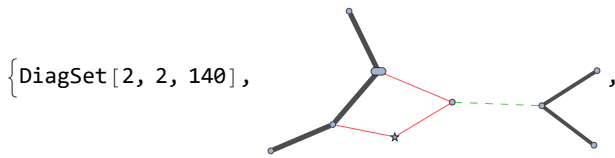

$$\begin{aligned} & \frac{1}{r} \left( \frac{1}{\vec{S}_1} \times \vec{v}_1 \cdot \vec{v}_2 \hat{n} \cdot \vec{a}_1 + \vec{S}_1 \times \vec{a}_1 \cdot \vec{v}_2 \hat{n} \cdot \vec{a}_1 + \vec{S}_1 \times \vec{v}_1 \cdot \vec{a}_2 \hat{n} \cdot \vec{a}_1 - \hat{n} \times \vec{S}_1 \cdot \vec{v}_1 \hat{n} \cdot \vec{a}_2 \hat{n} \cdot \vec{a}_1 - \hat{n} \times \vec{S}_1 \cdot \vec{v}_1 \hat{n} \cdot \vec{v}_2 \hat{n} \cdot \vec{a}_1 - \right. \\ & \hat{n} \times \vec{S}_1 \cdot \vec{a}_1 \hat{n} \cdot \vec{v}_2 \hat{n} \cdot \vec{a}_1 - \frac{2}{3} \vec{S}_1 \times \vec{v}_1 \cdot \vec{a}_1 \hat{n} \cdot \vec{a}_2 - \frac{2}{3} \frac{1}{\vec{S}_1} \times \vec{a}_1 \cdot \vec{v}_2 \hat{n} \cdot \vec{v}_1 - \frac{1}{3} \frac{1}{\vec{S}_1} \times \vec{v}_1 \cdot \vec{a}_2 \hat{n} \cdot \vec{v}_1 - \frac{1}{3} \frac{2}{\vec{S}_1} \times \vec{v}_1 \cdot \vec{v}_2 \hat{n} \cdot \vec{v}_1 - \\ & \frac{1}{3} \vec{S}_1 \times \frac{1}{\vec{a}_1} \cdot \vec{v}_2 \hat{n} \cdot \vec{v}_1 - \frac{1}{3} \vec{S}_1 \times \vec{a}_1 \cdot \vec{a}_2 \hat{n} \cdot \vec{v}_1 - \frac{1}{3} \hat{n} \times \vec{S}_1 \cdot \vec{v}_1 \hat{n} \cdot \vec{a}_2 \hat{n} \cdot \vec{v}_1 - \frac{1}{3} \hat{n} \times \vec{S}_1 \cdot \vec{a}_1 \hat{n} \cdot \vec{a}_2 \hat{n} \cdot \vec{v}_1 - \\ & \frac{1}{3} \frac{1}{\vec{S}_1} \times \vec{v}_1 \cdot \vec{a}_1 \hat{n} \cdot \vec{v}_2 + \frac{1}{3} \vec{S}_1 \times \vec{v}_1 \cdot \frac{1}{\vec{a}_1} \hat{n} \cdot \vec{v}_2 - \frac{2}{3} \hat{n} \times \vec{S}_1 \cdot \vec{a}_1 \hat{n} \cdot \vec{v}_1 \hat{n} \cdot \vec{v}_2 - \frac{1}{3} \hat{n} \times \vec{S}_1 \cdot \vec{v}_1 \hat{n} \cdot \vec{v}_1 \hat{n} \cdot \vec{v}_2 - \\ & \frac{1}{3} \hat{n} \times \vec{S}_1 \cdot \frac{1}{\vec{a}_1} \hat{n} \cdot \vec{v}_1 \hat{n} \cdot \vec{v}_2 - \hat{n} \times \vec{S}_1 \cdot \vec{v}_1 \vec{a}_1 \cdot \vec{a}_2 - \hat{n} \times \vec{S}_1 \cdot \vec{v}_1 \vec{a}_1 \cdot \vec{v}_2 - \hat{n} \times \vec{S}_1 \cdot \vec{a}_1 \vec{a}_1 \cdot \vec{v}_2 + \frac{5}{3} \hat{n} \times \vec{S}_1 \cdot \vec{v}_1 \vec{v}_1 \cdot \vec{a}_2 + \\ & \frac{5}{3} \hat{n} \times \vec{S}_1 \cdot \vec{a}_1 \vec{v}_1 \cdot \vec{a}_2 + \frac{10}{3} \hat{n} \times \vec{S}_1 \cdot \vec{a}_1 \vec{v}_1 \cdot \vec{v}_2 + \frac{5}{3} \hat{n} \times \vec{S}_1 \cdot \vec{v}_1 \vec{v}_1 \cdot \vec{v}_2 + \frac{5}{3} \hat{n} \times \vec{S}_1 \cdot \frac{1}{\vec{a}_1} \vec{v}_1 \cdot \vec{v}_2 \Big) m_1 m_2 G^2 + \frac{1}{r^2} \\ & \left( -\frac{1}{3} \vec{S}_1 \times \vec{v}_1 \cdot \vec{a}_2 (\hat{n} \cdot \vec{v}_1)^2 + \frac{4}{3} \hat{n} \times \vec{S}_1 \cdot \vec{v}_1 \hat{n} \cdot \vec{a}_2 (\hat{n} \cdot \vec{v}_1)^2 + 2 \hat{n} \times \vec{S}_1 \cdot \vec{v}_1 \hat{n} \cdot \vec{v}_2 (\hat{n} \cdot \vec{v}_1)^2 + 2 \hat{n} \times \vec{S}_1 \cdot \vec{a}_1 \hat{n} \cdot \vec{v}_2 (\hat{n} \cdot \vec{v}_1)^2 - \right. \\ & \frac{4}{3} \hat{n} \times \vec{S}_1 \cdot \vec{v}_1 (\hat{n} \cdot \vec{v}_2)^2 \hat{n} \cdot \vec{v}_1 - \frac{4}{3} \hat{n} \times \vec{S}_1 \cdot \vec{a}_1 (\hat{n} \cdot \vec{v}_2)^2 \hat{n} \cdot \vec{v}_1 - \vec{S}_1 \times \vec{v}_1 \cdot \vec{v}_2 \hat{n} \cdot \vec{a}_1 \hat{n} \cdot \vec{v}_1 - \frac{1}{3} \frac{1}{\vec{S}_1} \times \vec{v}_1 \cdot \vec{v}_2 \hat{n} \cdot \vec{v}_2 \hat{n} \cdot \vec{v}_1 - \\ & \frac{1}{3} \vec{S}_1 \times \vec{a}_1 \cdot \vec{v}_2 \hat{n} \cdot \vec{v}_2 \hat{n} \cdot \vec{v}_1 + \vec{S}_1 \times \vec{v}_1 \cdot \vec{a}_1 \hat{n} \cdot \vec{v}_2 \hat{n} \cdot \vec{v}_1 + 4 \hat{n} \times \vec{S}_1 \cdot \vec{v}_1 \hat{n} \cdot \vec{a}_1 \hat{n} \cdot \vec{v}_2 \hat{n} \cdot \vec{v}_1 + 2 \hat{n} \times \vec{S}_1 \cdot \vec{v}_1 \vec{a}_1 \cdot \vec{v}_2 \hat{n} \cdot \vec{v}_1 - \\ & \frac{5}{3} \hat{n} \times \vec{S}_1 \cdot \vec{v}_1 \vec{v}_1 \cdot \vec{a}_2 \hat{n} \cdot \vec{v}_1 - 4 \hat{n} \times \vec{S}_1 \cdot \vec{v}_1 \vec{v}_1 \cdot \vec{v}_2 \hat{n} \cdot \vec{v}_1 - 4 \hat{n} \times \vec{S}_1 \cdot \vec{a}_1 \vec{v}_1 \cdot \vec{v}_2 \hat{n} \cdot \vec{v}_1 + \frac{1}{3} \hat{n} \times \vec{S}_1 \cdot \vec{v}_1 \vec{v}_2 \cdot \vec{v}_2 \hat{n} \cdot \vec{v}_1 + \\ & \frac{1}{3} \hat{n} \times \vec{S}_1 \cdot \vec{a}_1 \vec{v}_2 \cdot \vec{v}_2 \hat{n} \cdot \vec{v}_1 - \frac{4}{3} \vec{S}_1 \times \vec{v}_1 \cdot \vec{a}_1 (\hat{n} \cdot \vec{v}_2)^2 - 4 \hat{n} \times \vec{S}_1 \cdot \vec{v}_1 \hat{n} \cdot \vec{a}_1 (\hat{n} \cdot \vec{v}_2)^2 + 3 \vec{S}_1 \times \vec{v}_1 \cdot \vec{v}_2 \hat{n} \cdot \vec{a}_1 \hat{n} \cdot \vec{v}_2 - \\ & \left. \hat{n} \times \vec{S}_1 \cdot \vec{v}_1 \hat{n} \cdot \vec{v}_2 \vec{a}_1 \cdot \vec{v}_2 - \vec{S}_1 \times \vec{v}_1 \cdot \vec{v}_2 \vec{v}_1 \cdot \vec{a}_1 + 2 \hat{n} \times \vec{S}_1 \cdot \vec{v}_1 \hat{n} \cdot \vec{v}_2 \vec{v}_1 \cdot \vec{a}_1 + \frac{2}{3} \vec{S}_1 \times \vec{v}_1 \cdot \vec{a}_2 \vec{v}_1 \cdot \vec{v}_1 - \right. \end{aligned}$$

$$\begin{aligned}
& \frac{7}{3} \hat{n} \times \vec{S}_1 \cdot \vec{v}_1 \hat{n} \cdot \vec{a}_2 \vec{v}_1 \cdot \vec{v}_1 - 2 \hat{n} \times \vec{S}_1 \cdot \vec{v}_1 \hat{n} \cdot \vec{v}_2 \vec{v}_1 \cdot \vec{v}_1 - 2 \hat{n} \times \vec{S}_1 \cdot \vec{a}_1 \hat{n} \cdot \vec{v}_2 \vec{v}_1 \cdot \vec{v}_1 - \frac{4}{3} \vec{S}_1 \times \vec{v}_1 \cdot \vec{v}_2 \vec{v}_1 \cdot \vec{v}_2 - \\
& \frac{4}{3} \vec{S}_1 \times \vec{a}_1 \cdot \vec{v}_2 \vec{v}_1 \cdot \vec{v}_2 + \vec{S}_1 \times \vec{v}_1 \cdot \vec{a}_1 \vec{v}_1 \cdot \vec{v}_2 - 4 \hat{n} \times \vec{S}_1 \cdot \vec{v}_1 \hat{n} \cdot \vec{a}_1 \vec{v}_1 \cdot \vec{v}_2 + \frac{11}{3} \hat{n} \times \vec{S}_1 \cdot \vec{v}_1 \hat{n} \cdot \vec{v}_2 \vec{v}_1 \cdot \vec{v}_2 + \\
& \frac{11}{3} \hat{n} \times \vec{S}_1 \cdot \vec{a}_1 \hat{n} \cdot \vec{v}_2 \vec{v}_1 \cdot \vec{v}_2 + \frac{2}{3} \vec{S}_1 \times \vec{v}_1 \cdot \vec{a}_1 \vec{v}_2 \cdot \vec{v}_2 + \hat{n} \times \vec{S}_1 \cdot \vec{v}_1 \hat{n} \cdot \vec{a}_1 \vec{v}_2 \cdot \vec{v}_2 \Big) m_1 m_2 G^2 + \\
& \frac{1}{r^3} \left( \frac{1}{3} \vec{S}_1 \times \vec{v}_1 \cdot \vec{v}_2 (\hat{n} \cdot \vec{v}_1)^3 - 5 \hat{n} \times \vec{S}_1 \cdot \vec{v}_1 \hat{n} \cdot \vec{v}_2 (\hat{n} \cdot \vec{v}_1)^3 + 8 \hat{n} \times \vec{S}_1 \cdot \vec{v}_1 (\hat{n} \cdot \vec{v}_2)^2 (\hat{n} \cdot \vec{v}_1)^2 - \right. \\
& \frac{8}{3} \vec{S}_1 \times \vec{v}_1 \cdot \vec{v}_2 \hat{n} \cdot \vec{v}_2 (\hat{n} \cdot \vec{v}_1)^2 + 7 \hat{n} \times \vec{S}_1 \cdot \vec{v}_1 \vec{v}_1 \cdot \vec{v}_2 (\hat{n} \cdot \vec{v}_1)^2 - \frac{4}{3} \hat{n} \times \vec{S}_1 \cdot \vec{v}_1 \vec{v}_2 \cdot \vec{v}_2 (\hat{n} \cdot \vec{v}_1)^2 - \\
& \vec{S}_1 \times \vec{v}_1 \cdot \vec{v}_2 \vec{v}_1 \cdot \vec{v}_1 \hat{n} \cdot \vec{v}_1 + 7 \hat{n} \times \vec{S}_1 \cdot \vec{v}_1 \hat{n} \cdot \vec{v}_2 \vec{v}_1 \cdot \vec{v}_1 \hat{n} \cdot \vec{v}_1 + \frac{7}{3} \vec{S}_1 \times \vec{v}_1 \cdot \vec{v}_2 \vec{v}_1 \cdot \vec{v}_2 \hat{n} \cdot \vec{v}_1 - \\
& \frac{28}{3} \hat{n} \times \vec{S}_1 \cdot \vec{v}_1 \hat{n} \cdot \vec{v}_2 \vec{v}_1 \cdot \vec{v}_2 \hat{n} \cdot \vec{v}_1 + \frac{5}{3} \hat{n} \times \vec{S}_1 \cdot \vec{v}_1 (\vec{v}_1 \cdot \vec{v}_2)^2 - \frac{28}{3} \hat{n} \times \vec{S}_1 \cdot \vec{v}_1 (\hat{n} \cdot \vec{v}_2)^2 \vec{v}_1 \cdot \vec{v}_1 + \\
& \left. \frac{11}{3} \vec{S}_1 \times \vec{v}_1 \cdot \vec{v}_2 \hat{n} \cdot \vec{v}_2 \vec{v}_1 \cdot \vec{v}_1 - \hat{n} \times \vec{S}_1 \cdot \vec{v}_1 \vec{v}_1 \cdot \vec{v}_1 \vec{v}_1 \cdot \vec{v}_2 + \frac{7}{3} \hat{n} \times \vec{S}_1 \cdot \vec{v}_1 \vec{v}_1 \cdot \vec{v}_1 \vec{v}_2 \cdot \vec{v}_2 \right) m_1 m_2 G^2 \Big\}
\end{aligned}$$

{DiagSet[2, 2, 141],

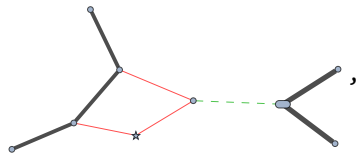

$$\begin{aligned}
& \frac{1}{r} G^2 \left( -\frac{1}{3} \hat{n} \times \vec{a}_1 \cdot \vec{S}_1 (\hat{n} \cdot \vec{v}_2)^2 + \frac{1}{3} \hat{n} \times \vec{S}_1 \cdot \vec{v}_1 (\hat{n} \cdot \vec{v}_2)^2 - \frac{2}{3} \hat{n} \times \vec{a}_1 \cdot \vec{S}_1 (\hat{n} \cdot \vec{v}_2)^2 + \frac{1}{3} \vec{a}_1 \times \vec{S}_1 \cdot \vec{v}_2 \hat{n} \cdot \vec{v}_2 - \right. \\
& \frac{1}{3} \vec{S}_1 \times \vec{v}_1 \cdot \vec{v}_2 \hat{n} \cdot \vec{v}_2 + \frac{2}{3} \vec{a}_1 \times \vec{S}_1 \cdot \vec{v}_2 \hat{n} \cdot \vec{v}_2 + \frac{2}{3} \vec{a}_1 \times \vec{a}_2 \cdot \vec{S}_1 \hat{n} \cdot \vec{v}_2 + \frac{2}{3} \vec{a}_2 \times \vec{S}_1 \cdot \vec{v}_1 \hat{n} \cdot \vec{v}_2 + \frac{2}{3} \hat{n} \times \vec{S}_1 \cdot \vec{v}_1 \hat{n} \cdot \vec{a}_2 \hat{n} \cdot \vec{v}_2 - \\
& \frac{2}{3} \hat{n} \times \vec{a}_1 \cdot \vec{S}_1 \hat{n} \cdot \vec{a}_2 \hat{n} \cdot \vec{v}_2 + \frac{1}{12} \vec{a}_2 \times \vec{S}_1 \cdot \vec{v}_1 \hat{n} \cdot \vec{a}_1 - \frac{4}{3} \vec{S}_1 \times \vec{v}_1 \cdot \vec{v}_2 \hat{n} \cdot \vec{a}_2 - \frac{1}{3} \vec{a}_1 \times \vec{S}_1 \cdot \vec{v}_1 \hat{n} \cdot \vec{a}_2 + \frac{4}{3} \vec{a}_1 \times \vec{S}_1 \cdot \vec{v}_2 \hat{n} \cdot \vec{a}_2 - \\
& \frac{2}{3} \hat{n} \times \vec{S}_1 \cdot \vec{v}_1 \hat{n} \cdot \vec{a}_1 \hat{n} \cdot \vec{a}_2 - \frac{7}{12} \vec{a}_1 \times \vec{a}_2 \cdot \vec{S}_1 \hat{n} \cdot \vec{v}_1 - \frac{7}{12} \vec{a}_2 \times \vec{S}_1 \cdot \vec{v}_1 \hat{n} \cdot \vec{v}_1 - \frac{4}{3} \hat{n} \times \vec{S}_1 \cdot \vec{v}_1 \hat{n} \cdot \vec{a}_2 \hat{n} \cdot \vec{v}_1 + \\
& \frac{4}{3} \hat{n} \times \vec{a}_1 \cdot \vec{S}_1 \hat{n} \cdot \vec{a}_2 \hat{n} \cdot \vec{v}_1 + 3 \hat{n} \times \vec{S}_1 \cdot \vec{v}_2 \vec{a}_2 \cdot \vec{v}_2 - \frac{5}{12} \hat{n} \times \vec{S}_1 \cdot \vec{v}_1 \vec{a}_1 \cdot \vec{a}_2 + 3 \hat{n} \times \vec{S}_1 \cdot \vec{v}_2 \vec{a}_2 \cdot \vec{a}_2 - \\
& \frac{1}{12} \hat{n} \times \vec{S}_1 \cdot \vec{v}_1 \vec{a}_2 \cdot \vec{v}_1 + \frac{1}{12} \hat{n} \times \vec{a}_1 \cdot \vec{S}_1 \vec{a}_2 \cdot \vec{v}_1 + \frac{2}{3} \hat{n} \times \vec{S}_1 \cdot \vec{v}_1 \vec{a}_2 \cdot \vec{v}_2 - 3 \hat{n} \times \vec{S}_1 \cdot \vec{v}_2 \vec{a}_2 \cdot \vec{v}_2 - \frac{2}{3} \hat{n} \times \vec{a}_1 \cdot \vec{S}_1 \vec{a}_2 \cdot \vec{v}_2 + \\
& \left. 3 \hat{n} \times \vec{a}_2 \cdot \vec{S}_1 \vec{a}_2 \cdot \vec{v}_2 + \frac{2}{3} \hat{n} \times \vec{a}_1 \cdot \vec{S}_1 \vec{v}_2 \cdot \vec{v}_2 - \frac{2}{3} \hat{n} \times \vec{S}_1 \cdot \vec{v}_1 \vec{v}_2 \cdot \vec{v}_2 + \frac{4}{3} \hat{n} \times \vec{a}_1 \cdot \vec{S}_1 \vec{v}_2 \cdot \vec{v}_2 + \frac{3}{2} \hat{n} \times \vec{a}_2 \cdot \vec{S}_1 \vec{v}_2 \cdot \vec{v}_2 \right) m_2^2 + \\
& \frac{1}{r^2} G^2 \left( \frac{2}{3} \hat{n} \times \vec{S}_1 \cdot \vec{v}_1 (\hat{n} \cdot \vec{v}_2)^3 - \frac{2}{3} \hat{n} \times \vec{a}_1 \cdot \vec{S}_1 (\hat{n} \cdot \vec{v}_2)^3 - \vec{S}_1 \times \vec{v}_1 \cdot \vec{v}_2 (\hat{n} \cdot \vec{v}_2)^2 - \frac{1}{3} \vec{a}_1 \times \vec{S}_1 \cdot \vec{v}_1 (\hat{n} \cdot \vec{v}_2)^2 + \right. \\
& \vec{a}_1 \times \vec{S}_1 \cdot \vec{v}_2 (\hat{n} \cdot \vec{v}_2)^2 - \frac{4}{3} \hat{n} \times \vec{S}_1 \cdot \vec{v}_1 \hat{n} \cdot \vec{a}_1 (\hat{n} \cdot \vec{v}_2)^2 - \frac{8}{3} \hat{n} \times \vec{S}_1 \cdot \vec{v}_1 \hat{n} \cdot \vec{v}_1 (\hat{n} \cdot \vec{v}_2)^2 + \frac{8}{3} \hat{n} \times \vec{a}_1 \cdot \vec{S}_1 \hat{n} \cdot \vec{v}_1 (\hat{n} \cdot \vec{v}_2)^2 + \\
& \frac{2}{3} \vec{S}_1 \times \vec{v}_1 \cdot \vec{v}_2 \hat{n} \cdot \vec{a}_1 \hat{n} \cdot \vec{v}_2 + \frac{4}{3} \vec{S}_1 \times \vec{v}_1 \cdot \vec{v}_2 \hat{n} \cdot \vec{v}_1 \hat{n} \cdot \vec{v}_2 - \frac{4}{3} \vec{a}_1 \times \vec{S}_1 \cdot \vec{v}_2 \hat{n} \cdot \vec{v}_1 \hat{n} \cdot \vec{v}_2 + \frac{1}{6} \vec{a}_2 \times \vec{S}_1 \cdot \vec{v}_1 \hat{n} \cdot \vec{v}_1 \hat{n} \cdot \vec{v}_2 - \\
& \frac{8}{3} \hat{n} \times \vec{S}_1 \cdot \vec{v}_1 \hat{n} \cdot \vec{a}_2 \hat{n} \cdot \vec{v}_1 \hat{n} \cdot \vec{v}_2 + \frac{2}{3} \hat{n} \times \vec{S}_1 \cdot \vec{v}_1 \vec{a}_1 \cdot \vec{v}_2 \hat{n} \cdot \vec{v}_2 - \frac{5}{6} \hat{n} \times \vec{S}_1 \cdot \vec{v}_1 \vec{a}_2 \cdot \vec{v}_1 \hat{n} \cdot \vec{v}_2 - 6 \hat{n} \times \vec{S}_1 \cdot \vec{v}_2 \vec{a}_2 \cdot \vec{v}_2 \hat{n} \cdot \vec{v}_2 + \\
& \frac{4}{3} \hat{n} \times \vec{S}_1 \cdot \vec{v}_1 \vec{v}_1 \cdot \vec{v}_2 \hat{n} \cdot \vec{v}_2 - \frac{4}{3} \hat{n} \times \vec{a}_1 \cdot \vec{S}_1 \vec{v}_1 \cdot \vec{v}_2 \hat{n} \cdot \vec{v}_2 - \hat{n} \times \vec{S}_1 \cdot \vec{v}_1 \vec{v}_2 \cdot \vec{v}_2 \hat{n} \cdot \vec{v}_2 + \hat{n} \times \vec{a}_1 \cdot \vec{S}_1 \vec{v}_2 \cdot \vec{v}_2 \hat{n} \cdot \vec{v}_2 + \\
& 3 \hat{n} \times \vec{a}_2 \cdot \vec{S}_1 \vec{v}_2 \cdot \vec{v}_2 \hat{n} \cdot \vec{v}_2 - \frac{1}{6} \vec{a}_2 \times \vec{S}_1 \cdot \vec{v}_1 (\hat{n} \cdot \vec{v}_1)^2 + \frac{8}{3} \hat{n} \times \vec{S}_1 \cdot \vec{v}_1 \hat{n} \cdot \vec{a}_2 (\hat{n} \cdot \vec{v}_1)^2 + \frac{7}{6} \vec{S}_1 \times \vec{v}_1 \cdot \vec{v}_2 \hat{n} \cdot \vec{a}_2 \hat{n} \cdot \vec{v}_1 - \\
& \frac{1}{3} \vec{S}_1 \times \vec{v}_1 \cdot \vec{v}_2 \vec{a}_1 \cdot \vec{v}_2 + \frac{1}{6} \vec{S}_1 \times \vec{v}_1 \cdot \vec{v}_2 \vec{a}_2 \cdot \vec{v}_1 + \frac{1}{6} \hat{n} \times \vec{S}_1 \cdot \vec{v}_1 \hat{n} \cdot \vec{v}_1 \vec{a}_2 \cdot \vec{v}_1 + 3 \vec{S}_1 \times \vec{v}_1 \cdot \vec{v}_2 \vec{a}_2 \cdot \vec{v}_2 - \\
& \left. \frac{4}{3} \hat{n} \times \vec{S}_1 \cdot \vec{v}_1 \hat{n} \cdot \vec{v}_1 \vec{a}_2 \cdot \vec{v}_2 + 6 \hat{n} \times \vec{S}_1 \cdot \vec{v}_2 \hat{n} \cdot \vec{v}_1 \vec{a}_2 \cdot \vec{v}_2 + \frac{1}{12} \vec{a}_2 \times \vec{S}_1 \cdot \vec{v}_1 \vec{v}_1 \cdot \vec{v}_1 - \frac{2}{3} \hat{n} \times \vec{S}_1 \cdot \vec{v}_1 \hat{n} \cdot \vec{a}_2 \vec{v}_1 \cdot \vec{v}_1 - \right.
\end{aligned}$$

$$\begin{aligned}
 & \frac{2}{3} \vec{S}_1 \times \vec{v}_1 \cdot \vec{v}_2 \vec{v}_1 \cdot \vec{v}_2 + \frac{2}{3} \vec{a}_1 \times \vec{S}_1 \cdot \vec{v}_2 \vec{v}_1 \cdot \vec{v}_2 - \frac{5}{6} \vec{a}_2 \times \vec{S}_1 \cdot \vec{v}_1 \vec{v}_1 \cdot \vec{v}_2 + \frac{13}{6} \hat{n} \times \vec{S}_1 \cdot \vec{v}_1 \hat{n} \cdot \vec{a}_2 \vec{v}_1 \cdot \vec{v}_2 + \\
 & \frac{2}{3} \vec{a}_1 \times \vec{S}_1 \cdot \vec{v}_1 \vec{v}_2 \cdot \vec{v}_2 + \frac{3}{2} \vec{a}_2 \times \vec{S}_1 \cdot \vec{v}_1 \vec{v}_2 \cdot \vec{v}_2 - 3 \vec{a}_2 \times \vec{S}_1 \cdot \vec{v}_2 \vec{v}_2 \cdot \vec{v}_2 + \frac{4}{3} \hat{n} \times \vec{S}_1 \cdot \vec{v}_1 \hat{n} \cdot \vec{a}_1 \vec{v}_2 \cdot \vec{v}_2 + \\
 & 3 \hat{n} \times \vec{S}_1 \cdot \vec{v}_2 \hat{n} \cdot \vec{a}_2 \vec{v}_2 \cdot \vec{v}_2 + \frac{8}{3} \hat{n} \times \vec{S}_1 \cdot \vec{v}_1 \hat{n} \cdot \vec{v}_1 \vec{v}_2 \cdot \vec{v}_2 - \frac{8}{3} \hat{n} \times \vec{a}_1 \cdot \vec{S}_1 \hat{n} \cdot \vec{v}_1 \vec{v}_2 \cdot \vec{v}_2 - 3 \hat{n} \times \vec{a}_2 \cdot \vec{S}_1 \hat{n} \cdot \vec{v}_1 \vec{v}_2 \cdot \vec{v}_2 \Big) m_2^2 + \\
 & \frac{1}{r^3} G^2 \left( -4 \hat{n} \times \vec{S}_1 \cdot \vec{v}_1 \hat{n} \cdot \vec{v}_1 (\hat{n} \cdot \vec{v}_2)^3 + 8 \hat{n} \times \vec{S}_1 \cdot \vec{v}_1 (\hat{n} \cdot \vec{v}_1)^2 (\hat{n} \cdot \vec{v}_2)^2 + \frac{5}{2} \vec{S}_1 \times \vec{v}_1 \cdot \vec{v}_2 \hat{n} \cdot \vec{v}_1 (\hat{n} \cdot \vec{v}_2)^2 - \right. \\
 & \frac{4}{3} \hat{n} \times \vec{S}_1 \cdot \vec{v}_1 \vec{v}_1 \cdot \vec{v}_1 (\hat{n} \cdot \vec{v}_2)^2 + \frac{7}{2} \hat{n} \times \vec{S}_1 \cdot \vec{v}_1 \vec{v}_1 \cdot \vec{v}_2 (\hat{n} \cdot \vec{v}_2)^2 + 3 \hat{n} \times \vec{S}_1 \cdot \vec{v}_2 \vec{v}_2 \cdot \vec{v}_2 (\hat{n} \cdot \vec{v}_2)^2 - \\
 & \frac{8}{3} \vec{S}_1 \times \vec{v}_1 \cdot \vec{v}_2 (\hat{n} \cdot \vec{v}_1)^2 \hat{n} \cdot \vec{v}_2 + \frac{2}{3} \vec{S}_1 \times \vec{v}_1 \cdot \vec{v}_2 \vec{v}_1 \cdot \vec{v}_1 \hat{n} \cdot \vec{v}_2 - 2 \vec{S}_1 \times \vec{v}_1 \cdot \vec{v}_2 \vec{v}_1 \cdot \vec{v}_2 \hat{n} \cdot \vec{v}_2 - \\
 & \frac{16}{3} \hat{n} \times \vec{S}_1 \cdot \vec{v}_1 \hat{n} \cdot \vec{v}_1 \vec{v}_1 \cdot \vec{v}_2 \hat{n} \cdot \vec{v}_2 + 4 \hat{n} \times \vec{S}_1 \cdot \vec{v}_1 \hat{n} \cdot \vec{v}_1 \vec{v}_2 \cdot \vec{v}_2 \hat{n} \cdot \vec{v}_2 + \frac{2}{3} \hat{n} \times \vec{S}_1 \cdot \vec{v}_1 (\vec{v}_1 \cdot \vec{v}_2)^2 + \\
 & \frac{3}{2} \hat{n} \times \vec{S}_1 \cdot \vec{v}_2 (\vec{v}_2 \cdot \vec{v}_2)^2 + \frac{4}{3} \vec{S}_1 \times \vec{v}_1 \cdot \vec{v}_2 \hat{n} \cdot \vec{v}_1 \vec{v}_1 \cdot \vec{v}_2 - \frac{16}{3} \hat{n} \times \vec{S}_1 \cdot \vec{v}_1 (\hat{n} \cdot \vec{v}_1)^2 \vec{v}_2 \cdot \vec{v}_2 - \\
 & \left. \frac{3}{4} \vec{S}_1 \times \vec{v}_1 \cdot \vec{v}_2 \hat{n} \cdot \vec{v}_1 \vec{v}_2 \cdot \vec{v}_2 + \frac{4}{3} \hat{n} \times \vec{S}_1 \cdot \vec{v}_1 \vec{v}_1 \cdot \vec{v}_1 \vec{v}_2 \cdot \vec{v}_2 - \frac{1}{4} \hat{n} \times \vec{S}_1 \cdot \vec{v}_1 \vec{v}_1 \cdot \vec{v}_2 \vec{v}_2 \cdot \vec{v}_2 \right) m_2^2 + \\
 & G^2 \left( -\frac{2}{3} \log\left(\frac{r}{R_\theta}\right) \vec{a}_1 \times \vec{a}_2 \cdot \vec{S}_1 + \frac{11}{18} \vec{a}_1 \times \vec{a}_2 \cdot \vec{S}_1 + \frac{11}{9} \vec{a}_1 \times \vec{a}_2 \cdot \vec{S}_1 + \frac{11}{18} \vec{a}_2 \times \vec{S}_1 \cdot \vec{v}_1 - \frac{1}{3} \hat{n} \times \vec{a}_1 \cdot \vec{S}_1 \hat{n} \cdot \vec{a}_2 + \right. \\
 & \frac{1}{3} \hat{n} \times \vec{S}_1 \cdot \vec{v}_1 \hat{n} \cdot \vec{a}_2 - \frac{2}{3} \hat{n} \times \vec{a}_1 \cdot \vec{S}_1 \hat{n} \cdot \vec{a}_2 - \frac{4}{3} \vec{a}_1 \times \vec{a}_2 \cdot \vec{S}_1 \log\left(\frac{r}{R_\theta}\right) - \\
 & \left. \frac{2}{3} \vec{a}_2 \times \vec{S}_1 \cdot \vec{v}_1 \log\left(\frac{r}{R_\theta}\right) + \frac{\frac{1}{3} \vec{a}_1 \times \vec{a}_2 \cdot \vec{S}_1 + \frac{2}{3} \vec{a}_1 \times \vec{a}_2 \cdot \vec{S}_1 + \frac{1}{3} \vec{a}_2 \times \vec{S}_1 \cdot \vec{v}_1}{\epsilon_d} \right) m_2^2 \Big\}
 \end{aligned}$$

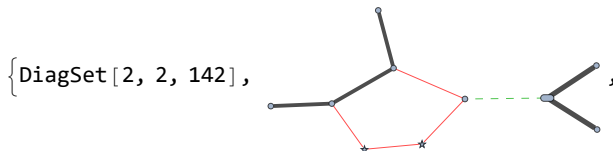

$$\begin{aligned}
 & \frac{1}{r} G^2 \left( -\frac{3}{8} \hat{n} \times \vec{S}_1 \cdot \vec{v}_2 (\hat{n} \cdot \vec{a}_2)^2 + \frac{1}{3} \vec{S}_1 \times \vec{v}_1 \cdot \vec{v}_2 \hat{n} \cdot \vec{a}_2 - \frac{1}{6} \vec{a}_1 \times \vec{S}_1 \cdot \vec{v}_2 \hat{n} \cdot \vec{a}_2 + \frac{1}{3} \vec{a}_2 \times \vec{S}_1 \cdot \vec{v}_1 \hat{n} \cdot \vec{a}_2 - \frac{1}{4} \vec{a}_2 \times \vec{S}_1 \cdot \vec{v}_2 \hat{n} \cdot \vec{a}_2 + \right. \\
 & \frac{1}{3} \hat{n} \times \vec{S}_1 \cdot \vec{v}_2 \hat{n} \cdot \vec{a}_1 \hat{n} \cdot \vec{a}_2 + \frac{2}{3} \hat{n} \times \vec{S}_1 \cdot \vec{v}_2 \hat{n} \cdot \vec{v}_1 \hat{n} \cdot \vec{a}_2 - \frac{2}{3} \hat{n} \times \vec{a}_2 \cdot \vec{S}_1 \hat{n} \cdot \vec{v}_1 \hat{n} \cdot \vec{a}_2 - \frac{1}{4} \hat{n} \times \vec{S}_1 \cdot \vec{v}_2 \hat{n} \cdot \vec{v}_2 \hat{n} \cdot \vec{a}_2 + \\
 & \frac{5}{4} \hat{n} \times \vec{a}_2 \cdot \vec{S}_1 \hat{n} \cdot \vec{v}_2 \hat{n} \cdot \vec{a}_2 - \frac{1}{6} \hat{n} \times \vec{a}_2 \cdot \vec{S}_1 (\hat{n} \cdot \vec{v}_1)^2 - \frac{7}{24} \hat{n} \times \vec{a}_2 \cdot \vec{S}_1 (\hat{n} \cdot \vec{v}_2)^2 + \frac{1}{24} \hat{n} \times \vec{S}_1 \cdot \vec{v}_2 (\hat{n} \cdot \vec{v}_2)^2 + \\
 & \frac{25}{24} \hat{n} \times \vec{a}_2 \cdot \vec{S}_1 (\hat{n} \cdot \vec{v}_2)^2 - \frac{1}{12} \vec{S}_1 \times \vec{v}_1 \cdot \vec{v}_2 \hat{n} \cdot \frac{1}{\vec{a}_2} + \frac{1}{12} \vec{a}_2 \times \vec{S}_1 \cdot \vec{v}_2 \hat{n} \cdot \vec{a}_1 + \frac{1}{6} \vec{a}_2 \times \vec{S}_1 \cdot \vec{v}_1 \hat{n} \cdot \vec{v}_1 - \\
 & \frac{1}{6} \vec{a}_2 \times \vec{S}_1 \cdot \vec{v}_2 \hat{n} \cdot \vec{v}_1 + \frac{1}{6} \vec{a}_2 \times \vec{S}_1 \cdot \vec{v}_2 \hat{n} \cdot \vec{v}_1 - \frac{1}{6} \hat{n} \times \vec{S}_1 \cdot \vec{v}_2 \hat{n} \cdot \frac{1}{\vec{a}_2} \hat{n} \cdot \vec{v}_1 - \frac{1}{4} \vec{a}_2 \times \vec{S}_1 \cdot \vec{v}_1 \hat{n} \cdot \vec{v}_2 + \frac{1}{6} \vec{a}_2 \times \vec{S}_1 \cdot \vec{v}_2 \hat{n} \cdot \vec{v}_2 + \\
 & \frac{1}{4} \vec{a}_1 \times \vec{a}_2 \cdot \vec{S}_1 \hat{n} \cdot \vec{v}_2 + \frac{1}{2} \vec{a}_2 \times \vec{S}_1 \cdot \vec{v}_1 \hat{n} \cdot \vec{v}_2 - \frac{11}{12} \vec{a}_2 \times \vec{S}_1 \cdot \vec{v}_2 \hat{n} \cdot \vec{v}_2 + \frac{1}{4} \hat{n} \times \vec{S}_1 \cdot \vec{v}_2 \hat{n} \cdot \frac{1}{\vec{a}_2} \hat{n} \cdot \vec{v}_2 - \\
 & \frac{1}{2} \hat{n} \times \vec{a}_2 \cdot \vec{S}_1 \hat{n} \cdot \vec{a}_1 \hat{n} \cdot \vec{v}_2 + \frac{1}{2} \hat{n} \times \vec{a}_2 \cdot \vec{S}_1 \hat{n} \cdot \vec{v}_1 \hat{n} \cdot \vec{v}_2 - \hat{n} \times \vec{a}_2 \cdot \vec{S}_1 \hat{n} \cdot \vec{v}_1 \hat{n} \cdot \vec{v}_2 + \frac{1}{12} \hat{n} \times \vec{S}_1 \cdot \vec{v}_2 \vec{a}_2 \cdot \vec{v}_1 + \\
 & \frac{1}{4} \hat{n} \times \vec{S}_1 \cdot \vec{v}_2 \vec{a}_2 \cdot \vec{v}_2 - \frac{1}{6} \hat{n} \times \vec{S}_1 \cdot \vec{v}_2 \vec{a}_1 \cdot \vec{a}_2 + \frac{1}{4} \hat{n} \times \vec{a}_2 \cdot \vec{S}_1 \vec{a}_1 \cdot \vec{v}_2 - \frac{3}{8} \hat{n} \times \vec{S}_1 \cdot \vec{v}_2 \vec{a}_2 \cdot \vec{a}_2 - \frac{1}{3} \hat{n} \times \vec{S}_1 \cdot \vec{v}_2 \vec{a}_2 \cdot \vec{v}_1 + \\
 & \left. \frac{1}{3} \hat{n} \times \vec{a}_2 \cdot \vec{S}_1 \vec{a}_2 \cdot \vec{v}_1 - \hat{n} \times \vec{S}_1 \cdot \vec{v}_2 \vec{a}_2 \cdot \vec{v}_2 + \frac{1}{2} \hat{n} \times \vec{a}_2 \cdot \vec{S}_1 \vec{a}_2 \cdot \vec{v}_2 + \frac{1}{12} \hat{n} \times \vec{a}_2 \cdot \vec{S}_1 \vec{v}_1 \cdot \vec{v}_1 - \frac{1}{4} \hat{n} \times \vec{a}_2 \cdot \vec{S}_1 \vec{v}_1 \cdot \vec{v}_2 + \right.
 \end{aligned}$$

$$\begin{aligned}
& \frac{1}{2} \hat{n} \times \vec{a}_2 \cdot \frac{1}{S_1} \vec{v}_1 \cdot \vec{v}_2 - \frac{1}{24} \hat{n} \times \vec{a}_2 \cdot \vec{S}_1 \cdot \vec{v}_2 \cdot \vec{v}_2 + \frac{13}{24} \hat{n} \times \vec{S}_1 \cdot \vec{v}_2 \vec{v}_2 \cdot \vec{v}_2 + \frac{1}{24} \hat{n} \times \vec{a}_2 \cdot \vec{S}_1 \vec{v}_2 \cdot \vec{v}_2 \Big) m_2^2 + \frac{1}{r^2} \\
& G^2 \left( \frac{1}{2} \hat{n} \times \vec{S}_1 \cdot \vec{v}_2 (\hat{n} \cdot \vec{v}_2)^3 + \frac{13}{6} \hat{n} \times \vec{a}_2 \cdot \vec{S}_1 (\hat{n} \cdot \vec{v}_2)^3 - \frac{1}{12} \vec{S}_1 \times \vec{v}_1 \cdot \vec{v}_2 (\hat{n} \cdot \vec{v}_2)^2 + \frac{1}{24} \vec{a}_1 \times \vec{S}_1 \cdot \vec{v}_2 (\hat{n} \cdot \vec{v}_2)^2 + \right. \\
& \frac{25}{24} \vec{a}_2 \times \vec{S}_1 \cdot \vec{v}_1 (\hat{n} \cdot \vec{v}_2)^2 - \frac{13}{8} \vec{a}_2 \times \vec{S}_1 \cdot \vec{v}_2 (\hat{n} \cdot \vec{v}_2)^2 - \frac{1}{6} \hat{n} \times \vec{S}_1 \cdot \vec{v}_2 \hat{n} \cdot \vec{a}_1 (\hat{n} \cdot \vec{v}_2)^2 - \frac{1}{3} \hat{n} \times \vec{S}_1 \cdot \vec{v}_2 \hat{n} \cdot \vec{v}_1 (\hat{n} \cdot \vec{v}_2)^2 - \\
& \frac{25}{6} \hat{n} \times \vec{a}_2 \cdot \vec{S}_1 \hat{n} \cdot \vec{v}_1 (\hat{n} \cdot \vec{v}_2)^2 + 2 \hat{n} \times \vec{a}_2 \cdot \vec{S}_1 (\hat{n} \cdot \vec{v}_1)^2 \hat{n} \cdot \vec{v}_2 + \frac{1}{4} \vec{S}_1 \times \vec{v}_1 \cdot \vec{v}_2 \hat{n} \cdot \vec{a}_2 \hat{n} \cdot \vec{v}_2 - \vec{a}_2 \times \vec{S}_1 \cdot \vec{v}_1 \hat{n} \cdot \vec{v}_1 \hat{n} \cdot \vec{v}_2 + \\
& \frac{11}{6} \vec{a}_2 \times \vec{S}_1 \cdot \vec{v}_2 \hat{n} \cdot \vec{v}_1 \hat{n} \cdot \vec{v}_2 + \hat{n} \times \vec{S}_1 \cdot \vec{v}_2 \hat{n} \cdot \vec{a}_2 \hat{n} \cdot \vec{v}_1 \hat{n} \cdot \vec{v}_2 + \frac{1}{12} \hat{n} \times \vec{S}_1 \cdot \vec{v}_2 \vec{a}_1 \cdot \vec{v}_2 \hat{n} \cdot \vec{v}_2 - \frac{1}{4} \hat{n} \times \vec{S}_1 \cdot \vec{v}_2 \vec{a}_2 \cdot \vec{v}_1 \hat{n} \cdot \vec{v}_2 - \\
& \frac{9}{4} \hat{n} \times \vec{S}_1 \cdot \vec{v}_2 \vec{a}_2 \cdot \vec{v}_2 \hat{n} \cdot \vec{v}_2 - \frac{1}{2} \hat{n} \times \vec{a}_2 \cdot \vec{S}_1 \vec{v}_1 \cdot \vec{v}_1 \hat{n} \cdot \vec{v}_2 + \frac{1}{6} \hat{n} \times \vec{S}_1 \cdot \vec{v}_2 \vec{v}_1 \cdot \vec{v}_2 \hat{n} \cdot \vec{v}_2 + \frac{25}{12} \hat{n} \times \vec{a}_2 \cdot \vec{S}_1 \vec{v}_1 \cdot \vec{v}_2 \hat{n} \cdot \vec{v}_2 + \\
& \frac{3}{2} \hat{n} \times \vec{S}_1 \cdot \vec{v}_2 \vec{v}_2 \cdot \vec{v}_2 \hat{n} \cdot \vec{v}_2 - \frac{1}{2} \hat{n} \times \vec{a}_2 \cdot \vec{S}_1 \vec{v}_2 \cdot \vec{v}_2 \hat{n} \cdot \vec{v}_2 - \frac{1}{6} \vec{a}_2 \times \vec{S}_1 \cdot \vec{v}_2 (\hat{n} \cdot \vec{v}_1)^2 - \frac{4}{3} \hat{n} \times \vec{S}_1 \cdot \vec{v}_2 \hat{n} \cdot \vec{a}_2 (\hat{n} \cdot \vec{v}_1)^2 - \\
& \frac{2}{3} \vec{S}_1 \times \vec{v}_1 \cdot \vec{v}_2 \hat{n} \cdot \vec{a}_2 \hat{n} \cdot \vec{v}_1 + \frac{1}{3} \vec{S}_1 \times \vec{v}_1 \cdot \vec{v}_2 \vec{a}_2 \cdot \vec{v}_1 + \frac{2}{3} \hat{n} \times \vec{S}_1 \cdot \vec{v}_2 \hat{n} \cdot \vec{v}_1 \vec{a}_2 \cdot \vec{v}_1 + \vec{S}_1 \times \vec{v}_1 \cdot \vec{v}_2 \vec{a}_2 \cdot \vec{v}_2 + \\
& 2 \hat{n} \times \vec{S}_1 \cdot \vec{v}_2 \hat{n} \cdot \vec{v}_1 \vec{a}_2 \cdot \vec{v}_2 + \frac{1}{12} \vec{a}_2 \times \vec{S}_1 \cdot \vec{v}_2 \vec{v}_1 \cdot \vec{v}_1 + \frac{1}{3} \hat{n} \times \vec{S}_1 \cdot \vec{v}_2 \hat{n} \cdot \vec{a}_2 \vec{v}_1 \cdot \vec{v}_1 + \frac{1}{2} \vec{a}_2 \times \vec{S}_1 \cdot \vec{v}_1 \vec{v}_1 \cdot \vec{v}_2 - \\
& \frac{11}{12} \vec{a}_2 \times \vec{S}_1 \cdot \vec{v}_2 \vec{v}_1 \cdot \vec{v}_2 - \frac{1}{4} \hat{n} \times \vec{S}_1 \cdot \vec{v}_2 \hat{n} \cdot \vec{a}_2 \vec{v}_1 \cdot \vec{v}_2 - \hat{n} \times \vec{a}_2 \cdot \vec{S}_1 \hat{n} \cdot \vec{v}_1 \vec{v}_1 \cdot \vec{v}_2 - \frac{13}{12} \vec{S}_1 \times \vec{v}_1 \cdot \vec{v}_2 \vec{v}_2 \cdot \vec{v}_2 + \\
& \frac{13}{24} \vec{a}_1 \times \vec{S}_1 \cdot \vec{v}_2 \vec{v}_2 \cdot \vec{v}_2 + \frac{1}{24} \vec{a}_2 \times \vec{S}_1 \cdot \vec{v}_1 \vec{v}_2 \cdot \vec{v}_2 - \frac{7}{8} \vec{a}_2 \times \vec{S}_1 \cdot \vec{v}_2 \vec{v}_2 \cdot \vec{v}_2 - \frac{13}{12} \hat{n} \times \vec{S}_1 \cdot \vec{v}_2 \hat{n} \cdot \vec{a}_1 \vec{v}_2 \cdot \vec{v}_2 + \\
& \frac{9}{4} \hat{n} \times \vec{S}_1 \cdot \vec{v}_2 \hat{n} \cdot \vec{a}_2 \vec{v}_2 \cdot \vec{v}_2 - \frac{13}{6} \hat{n} \times \vec{S}_1 \cdot \vec{v}_2 \hat{n} \cdot \vec{v}_1 \vec{v}_2 \cdot \vec{v}_2 - \frac{1}{12} \hat{n} \times \vec{a}_2 \cdot \vec{S}_1 \hat{n} \cdot \vec{v}_1 \vec{v}_2 \cdot \vec{v}_2 \Big) m_2^2 + \\
& \frac{1}{r^3} G^2 \left( \frac{23}{16} \hat{n} \times \vec{S}_1 \cdot \vec{v}_2 (\hat{n} \cdot \vec{v}_2)^4 - \frac{1}{2} \vec{S}_1 \times \vec{v}_1 \cdot \vec{v}_2 (\hat{n} \cdot \vec{v}_2)^3 - 3 \hat{n} \times \vec{S}_1 \cdot \vec{v}_2 \hat{n} \cdot \vec{v}_1 (\hat{n} \cdot \vec{v}_2)^3 + \right. \\
& \hat{n} \times \vec{S}_1 \cdot \vec{v}_2 (\hat{n} \cdot \vec{v}_1)^2 (\hat{n} \cdot \vec{v}_2)^2 + \frac{1}{3} \vec{S}_1 \times \vec{v}_1 \cdot \vec{v}_2 \hat{n} \cdot \vec{v}_1 (\hat{n} \cdot \vec{v}_2)^2 - \frac{1}{6} \hat{n} \times \vec{S}_1 \cdot \vec{v}_2 \vec{v}_1 \cdot \vec{v}_1 (\hat{n} \cdot \vec{v}_2)^2 + \\
& \frac{3}{2} \hat{n} \times \vec{S}_1 \cdot \vec{v}_2 \vec{v}_1 \cdot \vec{v}_2 (\hat{n} \cdot \vec{v}_2)^2 + \frac{23}{8} \hat{n} \times \vec{S}_1 \cdot \vec{v}_2 \vec{v}_2 \cdot \vec{v}_2 (\hat{n} \cdot \vec{v}_2)^2 - \frac{1}{6} \vec{S}_1 \times \vec{v}_1 \cdot \vec{v}_2 \vec{v}_1 \cdot \vec{v}_2 \hat{n} \cdot \vec{v}_2 - \\
& \frac{2}{3} \hat{n} \times \vec{S}_1 \cdot \vec{v}_2 \hat{n} \cdot \vec{v}_1 \vec{v}_1 \cdot \vec{v}_2 \hat{n} \cdot \vec{v}_2 - \frac{3}{2} \vec{S}_1 \times \vec{v}_1 \cdot \vec{v}_2 \vec{v}_2 \cdot \vec{v}_2 \hat{n} \cdot \vec{v}_2 - 6 \hat{n} \times \vec{S}_1 \cdot \vec{v}_2 \hat{n} \cdot \vec{v}_1 \vec{v}_2 \cdot \vec{v}_2 \hat{n} \cdot \vec{v}_2 + \\
& \frac{1}{12} \hat{n} \times \vec{S}_1 \cdot \vec{v}_2 (\vec{v}_1 \cdot \vec{v}_2)^2 - \frac{5}{16} \hat{n} \times \vec{S}_1 \cdot \vec{v}_2 (\vec{v}_2 \cdot \vec{v}_2)^2 + \frac{13}{3} \hat{n} \times \vec{S}_1 \cdot \vec{v}_2 (\hat{n} \cdot \vec{v}_1)^2 \vec{v}_2 \cdot \vec{v}_2 + \\
& \left. \frac{13}{6} \vec{S}_1 \times \vec{v}_1 \cdot \vec{v}_2 \hat{n} \cdot \vec{v}_1 \vec{v}_2 \cdot \vec{v}_2 - \frac{13}{12} \hat{n} \times \vec{S}_1 \cdot \vec{v}_2 \vec{v}_1 \cdot \vec{v}_1 \vec{v}_2 \cdot \vec{v}_2 + \frac{3}{2} \hat{n} \times \vec{S}_1 \cdot \vec{v}_2 \vec{v}_1 \cdot \vec{v}_2 \vec{v}_2 \cdot \vec{v}_2 \right) m_2^2 + \\
& G^2 r \left( \frac{1}{12} \log \left( \frac{r}{R_\theta} \right) \hat{n} \times \vec{a}_2 \cdot \vec{S}_1 - \frac{\hat{n} \times \vec{a}_2 \cdot \vec{S}_1}{24 \in_d} - \frac{17}{144} \hat{n} \times \vec{a}_2 \cdot \vec{S}_1 \right) m_2^2 + \\
& G^2 \left( \frac{1}{6} \log \left( \frac{r}{R_\theta} \right) \frac{1}{\vec{a}_2 \times \vec{S}_1} \cdot \vec{v}_1 - \frac{17}{72} \frac{1}{\vec{a}_2 \times \vec{S}_1} \cdot \vec{v}_1 + \frac{17}{72} \frac{1}{\vec{a}_2 \times \vec{S}_1} \cdot \vec{v}_2 - \frac{17}{144} \vec{a}_1 \times \frac{1}{\vec{a}_2} \cdot \vec{S}_1 + \frac{17}{72} \vec{a}_2 \times \frac{1}{\vec{a}_2} \cdot \vec{S}_1 - \right. \\
& \frac{17}{144} \vec{a}_2 \times \frac{1}{\vec{S}_1} \cdot \vec{v}_2 + \frac{1}{12} \hat{n} \times \vec{S}_1 \cdot \vec{v}_2 \hat{n} \cdot \frac{1}{\vec{a}_2} + \frac{1}{12} \hat{n} \times \vec{a}_2 \cdot \vec{S}_1 \hat{n} \cdot \frac{1}{\vec{a}_2} + \frac{1}{12} \hat{n} \times \vec{a}_2 \cdot \vec{S}_1 \hat{n} \cdot \vec{a}_1 - \frac{1}{12} \hat{n} \times \vec{a}_2 \cdot \vec{S}_1 \hat{n} \cdot \vec{a}_2 - \\
& \frac{1}{6} \hat{n} \times \vec{S}_1 \cdot \vec{v}_2 \hat{n} \cdot \vec{a}_2 + \frac{1}{3} \hat{n} \times \vec{a}_2 \cdot \vec{S}_1 \hat{n} \cdot \vec{a}_2 + \frac{1}{6} \hat{n} \times \vec{a}_2 \cdot \vec{S}_1 \hat{n} \cdot \vec{v}_1 - \frac{1}{4} \hat{n} \times \vec{a}_2 \cdot \vec{S}_1 \hat{n} \cdot \vec{v}_2 + \frac{1}{4} \hat{n} \times \vec{a}_2 \cdot \vec{S}_1 \hat{n} \cdot \vec{v}_2 - \\
& \frac{1}{6} \frac{1}{\vec{a}_2 \times \vec{S}_1} \cdot \vec{v}_2 \log \left( \frac{r}{R_\theta} \right) + \frac{1}{12} \vec{a}_1 \times \frac{1}{\vec{a}_2} \cdot \vec{S}_1 \log \left( \frac{r}{R_\theta} \right) - \frac{1}{6} \vec{a}_2 \times \frac{1}{\vec{a}_2} \cdot \vec{S}_1 \log \left( \frac{r}{R_\theta} \right) + \frac{1}{12} \vec{a}_2 \times \vec{S}_1 \cdot \vec{v}_2 \log \left( \frac{r}{R_\theta} \right) + \\
& \left. \frac{1}{\in_d} \left( -\frac{1}{12} \frac{1}{\vec{a}_2 \times \vec{S}_1} \cdot \vec{v}_1 + \frac{1}{12} \frac{1}{\vec{a}_2 \times \vec{S}_1} \cdot \vec{v}_2 - \frac{1}{24} \vec{a}_1 \times \frac{1}{\vec{a}_2} \cdot \vec{S}_1 + \frac{1}{12} \vec{a}_2 \times \frac{1}{\vec{a}_2} \cdot \vec{S}_1 - \frac{1}{24} \vec{a}_2 \times \vec{S}_1 \cdot \vec{v}_2 \right) \right) m_2^2 \Big\}
\end{aligned}$$

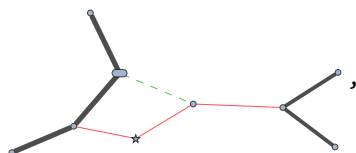

[illegible]

$$\begin{aligned}
& \left. \frac{3}{2} \hat{n} \times \vec{S}_1 \cdot \vec{v}_1 \hat{n} \cdot \vec{a}_2 \vec{v}_2 \cdot \vec{v}_2 + \frac{3}{2} \hat{n} \times \vec{S}_1 \cdot \vec{v}_1 \hat{n} \cdot \vec{v}_2 \vec{v}_2 \cdot \vec{v}_2 - \frac{3}{2} \hat{n} \times \vec{S}_1 \cdot \vec{a}_1 \hat{n} \cdot \vec{v}_2 \vec{v}_2 \cdot \vec{v}_2 \right) m_1 m_2 G^2 + \frac{1}{r^3} \\
& \left( 2 \hat{n} \times \vec{S}_1 \cdot \vec{v}_1 (\hat{n} \cdot \vec{v}_1)^4 + \frac{1}{3} \vec{S}_1 \times \vec{v}_1 \cdot \vec{v}_2 (\hat{n} \cdot \vec{v}_1)^3 - 2 \hat{n} \times \vec{S}_1 \cdot \vec{v}_1 \hat{n} \cdot \vec{v}_2 (\hat{n} \cdot \vec{v}_1)^3 - 4 \hat{n} \times \vec{S}_1 \cdot \vec{v}_1 (\hat{n} \cdot \vec{v}_2)^2 (\hat{n} \cdot \vec{v}_1)^2 + \right. \\
& \frac{4}{3} \vec{S}_1 \times \vec{v}_1 \cdot \vec{v}_2 \hat{n} \cdot \vec{v}_2 (\hat{n} \cdot \vec{v}_1)^2 - \frac{11}{2} \hat{n} \times \vec{S}_1 \cdot \vec{v}_1 \vec{v}_1 \cdot \vec{v}_1 (\hat{n} \cdot \vec{v}_1)^2 + \hat{n} \times \vec{S}_1 \cdot \vec{v}_1 \vec{v}_1 \cdot \vec{v}_2 (\hat{n} \cdot \vec{v}_1)^2 - \\
& \frac{1}{12} \hat{n} \times \vec{S}_1 \cdot \vec{v}_1 \vec{v}_2 \cdot \vec{v}_2 (\hat{n} \cdot \vec{v}_1)^2 - \vec{S}_1 \times \vec{v}_1 \cdot \vec{v}_2 \vec{v}_1 \cdot \vec{v}_1 \hat{n} \cdot \vec{v}_1 + 4 \hat{n} \times \vec{S}_1 \cdot \vec{v}_1 \hat{n} \cdot \vec{v}_2 \vec{v}_1 \cdot \vec{v}_1 \hat{n} \cdot \vec{v}_1 - \\
& \frac{2}{3} \vec{S}_1 \times \vec{v}_1 \cdot \vec{v}_2 \vec{v}_1 \cdot \vec{v}_2 \hat{n} \cdot \vec{v}_1 + \frac{8}{3} \hat{n} \times \vec{S}_1 \cdot \vec{v}_1 \hat{n} \cdot \vec{v}_2 \vec{v}_1 \cdot \vec{v}_2 \hat{n} \cdot \vec{v}_1 + \frac{3}{2} \hat{n} \times \vec{S}_1 \cdot \vec{v}_1 (\vec{v}_1 \cdot \vec{v}_1)^2 - \frac{1}{3} \hat{n} \times \vec{S}_1 \cdot \vec{v}_1 (\vec{v}_1 \cdot \vec{v}_2)^2 - \\
& \frac{3}{2} \hat{n} \times \vec{S}_1 \cdot \vec{v}_1 (\vec{v}_2 \cdot \vec{v}_2)^2 + \frac{32}{3} \hat{n} \times \vec{S}_1 \cdot \vec{v}_1 (\hat{n} \cdot \vec{v}_2)^2 \vec{v}_1 \cdot \vec{v}_1 - \frac{16}{3} \vec{S}_1 \times \vec{v}_1 \cdot \vec{v}_2 \hat{n} \cdot \vec{v}_2 \vec{v}_1 \cdot \vec{v}_1 - \hat{n} \times \vec{S}_1 \cdot \vec{v}_1 \vec{v}_1 \cdot \vec{v}_1 \vec{v}_1 \cdot \vec{v}_2 + \\
& \left. 6 \hat{n} \times \vec{S}_1 \cdot \vec{v}_1 (\hat{n} \cdot \vec{v}_2)^2 \vec{v}_2 \cdot \vec{v}_2 - 3 \vec{S}_1 \times \vec{v}_1 \cdot \vec{v}_2 \hat{n} \cdot \vec{v}_2 \vec{v}_2 \cdot \vec{v}_2 - \frac{23}{12} \hat{n} \times \vec{S}_1 \cdot \vec{v}_1 \vec{v}_1 \cdot \vec{v}_1 \vec{v}_2 \cdot \vec{v}_2 \right) m_1 m_2 G^2 + \\
& m_1 m_2 \left( -\frac{2}{3} \log\left(\frac{r}{R_\theta}\right) \vec{S}_1 \times \vec{v}_1 \cdot \vec{a}_1 + \frac{5}{18} \vec{S}_1 \times \vec{v}_1 \cdot \vec{a}_1 - \frac{5}{18} \vec{S}_1 \times \vec{a}_1 \cdot \vec{a}_1 - \frac{4}{3} \hat{n} \times \vec{S}_1 \cdot \vec{a}_1 \hat{n} \cdot \vec{a}_1 - \frac{2}{3} \hat{n} \times \vec{S}_1 \cdot \vec{v}_1 \hat{n} \cdot \vec{a}_1 - \right. \\
& \left. \frac{2}{3} \hat{n} \times \vec{S}_1 \cdot \vec{a}_1 \hat{n} \cdot \vec{a}_1 + \frac{2}{3} \vec{S}_1 \times \vec{a}_1 \cdot \vec{a}_1 \log\left(\frac{r}{R_\theta}\right) + \frac{\frac{1}{3} \vec{S}_1 \times \vec{v}_1 \cdot \vec{a}_1 - \frac{1}{3} \vec{S}_1 \times \vec{a}_1 \cdot \vec{a}_1}{\epsilon_d} \right) G^2 \}
\end{aligned}$$

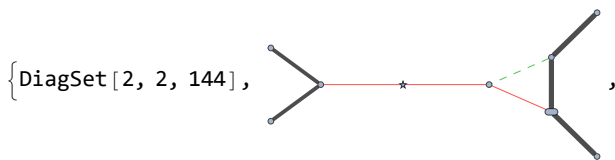

$$\begin{aligned}
& \frac{1}{r} \left( \frac{4}{3} \vec{S}_1 \times \vec{v}_1 \cdot \vec{v}_2 \hat{n} \cdot \vec{a}_1 + \frac{4}{3} \vec{S}_1 \times \vec{a}_1 \cdot \vec{v}_2 \hat{n} \cdot \vec{a}_1 - \vec{S}_1 \times \vec{v}_1 \cdot \vec{a}_2 \hat{n} \cdot \vec{a}_1 + 2 \hat{n} \times \vec{S}_1 \cdot \vec{v}_1 \hat{n} \cdot \vec{a}_2 \hat{n} \cdot \vec{a}_1 - \frac{8}{3} \hat{n} \times \vec{S}_1 \cdot \vec{v}_1 \hat{n} \cdot \vec{v}_2 \hat{n} \cdot \vec{a}_1 - \right. \\
& \frac{8}{3} \hat{n} \times \vec{S}_1 \cdot \vec{a}_1 \hat{n} \cdot \vec{v}_2 \hat{n} \cdot \vec{a}_1 + \frac{8}{3} \vec{S}_1 \times \vec{a}_1 \cdot \vec{v}_2 \hat{n} \cdot \vec{v}_1 - \vec{S}_1 \times \vec{v}_1 \cdot \vec{a}_2 \hat{n} \cdot \vec{v}_1 + \frac{4}{3} \vec{S}_1 \times \vec{v}_1 \cdot \vec{v}_2 \hat{n} \cdot \vec{v}_1 + \\
& \frac{4}{3} \vec{S}_1 \times \vec{a}_1 \cdot \vec{v}_2 \hat{n} \cdot \vec{v}_1 - \vec{S}_1 \times \vec{a}_1 \cdot \vec{a}_2 \hat{n} \cdot \vec{v}_1 + 2 \hat{n} \times \vec{S}_1 \cdot \vec{v}_1 \hat{n} \cdot \vec{a}_2 \hat{n} \cdot \vec{v}_1 + 2 \hat{n} \times \vec{S}_1 \cdot \vec{a}_1 \hat{n} \cdot \vec{a}_2 \hat{n} \cdot \vec{v}_1 - \\
& \frac{4}{3} \vec{S}_1 \times \vec{v}_1 \cdot \vec{a}_1 \hat{n} \cdot \vec{v}_2 - \frac{4}{3} \vec{S}_1 \times \vec{v}_1 \cdot \vec{a}_1 \hat{n} \cdot \vec{v}_2 - \frac{16}{3} \hat{n} \times \vec{S}_1 \cdot \vec{a}_1 \hat{n} \cdot \vec{v}_1 \hat{n} \cdot \vec{v}_2 - \frac{8}{3} \hat{n} \times \vec{S}_1 \cdot \vec{v}_1 \hat{n} \cdot \vec{v}_1 \hat{n} \cdot \vec{v}_2 - \\
& \frac{8}{3} \hat{n} \times \vec{S}_1 \cdot \vec{a}_1 \hat{n} \cdot \vec{v}_1 \hat{n} \cdot \vec{v}_2 - \hat{n} \times \vec{S}_1 \cdot \vec{v}_1 \vec{a}_1 \cdot \vec{a}_2 + \frac{4}{3} \hat{n} \times \vec{S}_1 \cdot \vec{v}_1 \vec{a}_1 \cdot \vec{v}_2 + \frac{4}{3} \hat{n} \times \vec{S}_1 \cdot \vec{a}_1 \vec{a}_1 \cdot \vec{v}_2 - \hat{n} \times \vec{S}_1 \cdot \vec{v}_1 \vec{v}_1 \cdot \vec{a}_2 - \\
& \left. \hat{n} \times \vec{S}_1 \cdot \vec{a}_1 \vec{v}_1 \cdot \vec{a}_2 + \frac{8}{3} \hat{n} \times \vec{S}_1 \cdot \vec{a}_1 \vec{v}_1 \cdot \vec{v}_2 + \frac{4}{3} \hat{n} \times \vec{S}_1 \cdot \vec{v}_1 \vec{v}_1 \cdot \vec{v}_2 + \frac{4}{3} \hat{n} \times \vec{S}_1 \cdot \vec{a}_1 \vec{v}_1 \cdot \vec{v}_2 \right) m_1 m_2 G^2 + \frac{1}{r^2} \\
& \left( -\frac{14}{3} \vec{S}_1 \times \vec{v}_1 \cdot \vec{v}_2 (\hat{n} \cdot \vec{v}_1)^2 - \frac{14}{3} \vec{S}_1 \times \vec{a}_1 \cdot \vec{v}_2 (\hat{n} \cdot \vec{v}_1)^2 + 2 \vec{S}_1 \times \vec{v}_1 \cdot \vec{a}_2 (\hat{n} \cdot \vec{v}_1)^2 - 8 \hat{n} \times \vec{S}_1 \cdot \vec{v}_1 \hat{n} \cdot \vec{a}_2 (\hat{n} \cdot \vec{v}_1)^2 + \right. \\
& \frac{56}{3} \hat{n} \times \vec{S}_1 \cdot \vec{v}_1 \hat{n} \cdot \vec{v}_2 (\hat{n} \cdot \vec{v}_1)^2 + \frac{56}{3} \hat{n} \times \vec{S}_1 \cdot \vec{a}_1 \hat{n} \cdot \vec{v}_2 (\hat{n} \cdot \vec{v}_1)^2 + 8 \hat{n} \times \vec{S}_1 \cdot \vec{v}_1 (\hat{n} \cdot \vec{v}_2)^2 \hat{n} \cdot \vec{v}_1 + \\
& 8 \hat{n} \times \vec{S}_1 \cdot \vec{a}_1 (\hat{n} \cdot \vec{v}_2)^2 \hat{n} \cdot \vec{v}_1 - 4 \vec{S}_1 \times \vec{v}_1 \cdot \vec{v}_2 \hat{n} \cdot \vec{a}_1 \hat{n} \cdot \vec{v}_1 - 4 \vec{S}_1 \times \vec{v}_1 \cdot \vec{v}_2 \hat{n} \cdot \vec{v}_2 \hat{n} \cdot \vec{v}_1 - 4 \vec{S}_1 \times \vec{a}_1 \cdot \vec{v}_2 \hat{n} \cdot \vec{v}_2 \hat{n} \cdot \vec{v}_1 + \\
& \frac{16}{3} \vec{S}_1 \times \vec{v}_1 \cdot \vec{a}_1 \hat{n} \cdot \vec{v}_2 \hat{n} \cdot \vec{v}_1 + 16 \hat{n} \times \vec{S}_1 \cdot \vec{v}_1 \hat{n} \cdot \vec{a}_1 \hat{n} \cdot \vec{v}_2 \hat{n} \cdot \vec{v}_1 - 4 \hat{n} \times \vec{S}_1 \cdot \vec{v}_1 \vec{a}_1 \cdot \vec{v}_2 \hat{n} \cdot \vec{v}_1 + \\
& 4 \hat{n} \times \vec{S}_1 \cdot \vec{v}_1 \vec{v}_1 \cdot \vec{a}_2 \hat{n} \cdot \vec{v}_1 - \frac{28}{3} \hat{n} \times \vec{S}_1 \cdot \vec{v}_1 \vec{v}_1 \cdot \vec{v}_2 \hat{n} \cdot \vec{v}_1 - \frac{28}{3} \hat{n} \times \vec{S}_1 \cdot \vec{a}_1 \vec{v}_1 \cdot \vec{v}_2 \hat{n} \cdot \vec{v}_1 - 2 \hat{n} \times \vec{S}_1 \cdot \vec{v}_1 \vec{v}_2 \cdot \vec{v}_2 \hat{n} \cdot \vec{v}_1 - \\
& 2 \hat{n} \times \vec{S}_1 \cdot \vec{a}_1 \vec{v}_2 \cdot \vec{v}_2 \hat{n} \cdot \vec{v}_1 + 8 \hat{n} \times \vec{S}_1 \cdot \vec{v}_1 \hat{n} \cdot \vec{a}_1 (\hat{n} \cdot \vec{v}_2)^2 - 4 \vec{S}_1 \times \vec{v}_1 \cdot \vec{v}_2 \hat{n} \cdot \vec{a}_1 \hat{n} \cdot \vec{v}_2 + 2 \vec{S}_1 \times \vec{v}_1 \cdot \vec{v}_2 \vec{a}_1 \cdot \vec{v}_2 - \\
& \left. 4 \hat{n} \times \vec{S}_1 \cdot \vec{v}_1 \hat{n} \cdot \vec{v}_2 \vec{a}_1 \cdot \vec{v}_2 + 2 \vec{S}_1 \times \vec{v}_1 \cdot \vec{v}_2 \vec{v}_1 \cdot \vec{a}_1 - 4 \hat{n} \times \vec{S}_1 \cdot \vec{v}_1 \hat{n} \cdot \vec{v}_2 \vec{v}_1 \cdot \vec{a}_1 + \frac{7}{3} \vec{S}_1 \times \vec{v}_1 \cdot \vec{v}_2 \vec{v}_1 \cdot \vec{v}_1 + \right.
\end{aligned}$$

$$\begin{aligned} & \frac{7}{3} \vec{S_1} \times \vec{a_1} \cdot \vec{v_2} \vec{v_1} \cdot \vec{v_1} - \vec{S_1} \times \vec{v_1} \cdot \vec{a_2} \vec{v_1} \cdot \vec{v_1} + 2 \hat{n} \times \vec{S_1} \cdot \vec{v_1} \hat{n} \cdot \vec{a_2} \vec{v_1} \cdot \vec{v_1} - \frac{14}{3} \hat{n} \times \vec{S_1} \cdot \vec{v_1} \hat{n} \cdot \vec{v_2} \vec{v_1} \cdot \vec{v_1} - \\ & \frac{14}{3} \hat{n} \times \vec{S_1} \cdot \vec{a_1} \hat{n} \cdot \vec{v_2} \vec{v_1} \cdot \vec{v_1} + 2 \vec{S_1} \times \vec{v_1} \cdot \vec{v_2} \vec{v_1} \cdot \vec{v_2} + 2 \vec{S_1} \times \vec{a_1} \cdot \vec{v_2} \vec{v_1} \cdot \vec{v_2} - \frac{8}{3} \vec{S_1} \times \vec{v_1} \cdot \vec{a_1} \vec{v_1} \cdot \vec{v_2} - \\ & 4 \hat{n} \times \vec{S_1} \cdot \vec{v_1} \hat{n} \cdot \vec{a_1} \vec{v_1} \cdot \vec{v_2} - 4 \hat{n} \times \vec{S_1} \cdot \vec{v_1} \hat{n} \cdot \vec{v_2} \vec{v_1} \cdot \vec{v_2} - 4 \hat{n} \times \vec{S_1} \cdot \vec{a_1} \hat{n} \cdot \vec{v_2} \vec{v_1} \cdot \vec{v_2} - 2 \hat{n} \times \vec{S_1} \cdot \vec{v_1} \hat{n} \cdot \vec{a_1} \vec{v_2} \cdot \vec{v_2} \Big) m_1 m_2 G^2 + \\ & \frac{1}{\rho^3} \Big( 8 \vec{S_1} \times \vec{v_1} \cdot \vec{v_2} (\hat{n} \cdot \vec{v_1})^3 - 48 \hat{n} \times \vec{S_1} \cdot \vec{v_1} \hat{n} \cdot \vec{v_2} (\hat{n} \cdot \vec{v_1})^3 - 48 \hat{n} \times \vec{S_1} \cdot \vec{v_1} (\hat{n} \cdot \vec{v_2})^2 (\hat{n} \cdot \vec{v_1})^2 + \\ & 16 \vec{S_1} \times \vec{v_1} \cdot \vec{v_2} \hat{n} \cdot \vec{v_2} (\hat{n} \cdot \vec{v_1})^2 + 24 \hat{n} \times \vec{S_1} \cdot \vec{v_1} \vec{v_1} \cdot \vec{v_2} (\hat{n} \cdot \vec{v_1})^2 + 8 \hat{n} \times \vec{S_1} \cdot \vec{v_1} \vec{v_2} \cdot \vec{v_2} (\hat{n} \cdot \vec{v_1})^2 - \\ & 6 \vec{S_1} \times \vec{v_1} \cdot \vec{v_2} \vec{v_1} \cdot \vec{v_1} \hat{n} \cdot \vec{v_1} + 24 \hat{n} \times \vec{S_1} \cdot \vec{v_1} \hat{n} \cdot \vec{v_2} \vec{v_1} \cdot \vec{v_1} \hat{n} \cdot \vec{v_1} - 8 \vec{S_1} \times \vec{v_1} \cdot \vec{v_2} \vec{v_1} \cdot \vec{v_2} \hat{n} \cdot \vec{v_1} + \\ & 32 \hat{n} \times \vec{S_1} \cdot \vec{v_1} \hat{n} \cdot \vec{v_2} \vec{v_1} \cdot \vec{v_2} \hat{n} \cdot \vec{v_1} - 4 \hat{n} \times \vec{S_1} \cdot \vec{v_1} (\vec{v_1} \cdot \vec{v_2})^2 + 8 \hat{n} \times \vec{S_1} \cdot \vec{v_1} (\hat{n} \cdot \vec{v_2})^2 \vec{v_1} \cdot \vec{v_1} - \\ & 4 \vec{S_1} \times \vec{v_1} \cdot \vec{v_2} \hat{n} \cdot \vec{v_2} \vec{v_1} \cdot \vec{v_1} - 6 \hat{n} \times \vec{S_1} \cdot \vec{v_1} \vec{v_1} \cdot \vec{v_1} \vec{v_1} \cdot \vec{v_2} - 2 \hat{n} \times \vec{S_1} \cdot \vec{v_1} \vec{v_1} \cdot \vec{v_1} \vec{v_2} \cdot \vec{v_2} \Big) m_1 m_2 G^2 \Big\} \end{aligned}$$

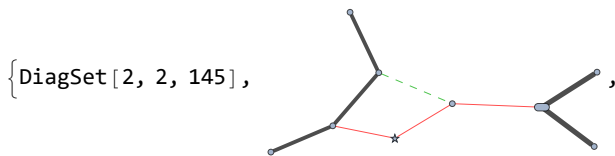

$$\begin{aligned} & \frac{1}{r} G^2 \left( \frac{8}{3} \hat{n} \times \vec{S}_1 \cdot \vec{V}_1 (\hat{n} \cdot \vec{a}_2)^2 - \frac{2}{3} \vec{S}_1 \times \vec{V}_1 \cdot \vec{V}_2 \hat{n} \cdot \vec{a}_2 + \frac{2}{3} \vec{a}_1 \times \vec{S}_1 \cdot \vec{V}_2 \hat{n} \cdot \vec{a}_2 - \frac{8}{3} \vec{a}_2 \times \vec{S}_1 \cdot \vec{V}_1 \hat{n} \cdot \vec{a}_2 + \frac{4}{3} \hat{n} \times \vec{S}_1 \cdot \vec{V}_1 \hat{n} \cdot \vec{V}_2 \hat{n} \cdot \vec{a}_2 - \right. \\ & \quad \frac{4}{3} \hat{n} \times \vec{a}_1 \cdot \vec{S}_1 \hat{n} \cdot \vec{V}_2 \hat{n} \cdot \vec{a}_2 + \frac{4}{3} \hat{n} \times \vec{a}_1 \cdot \vec{S}_1 (\hat{n} \cdot \vec{V}_2)^2 - \frac{4}{3} \hat{n} \times \vec{S}_1 \cdot \vec{V}_1 (\hat{n} \cdot \vec{V}_2)^2 + \frac{8}{3} \hat{n} \times \vec{a}_1 \cdot \vec{S}_1 (\hat{n} \cdot \vec{V}_2)^2 - \frac{4}{3} \frac{1}{\vec{a}_1 \times \vec{S}_1} \cdot \vec{V}_2 \\ & \quad \hat{n} \cdot \vec{V}_2 + \frac{4}{3} \frac{1}{\vec{S}_1 \times \vec{V}_1} \cdot \vec{V}_2 \hat{n} \cdot \vec{V}_2 - \frac{8}{3} \vec{a}_1 \times \vec{S}_1 \cdot \vec{V}_2 \hat{n} \cdot \vec{V}_2 - \frac{2}{3} \vec{a}_1 \times \vec{a}_2 \cdot \vec{S}_1 \hat{n} \cdot \vec{V}_2 - \frac{2}{3} \vec{a}_2 \times \vec{S}_1 \cdot \vec{V}_1 \hat{n} \cdot \vec{V}_2 - \frac{4}{3} \hat{n} \times \vec{S}_1 \cdot \vec{V}_1 \vec{a}_2 \cdot \vec{a}_2 + \\ & \quad \left. \frac{4}{3} \hat{n} \times \vec{S}_1 \cdot \vec{V}_1 \vec{a}_2 \cdot \vec{V}_2 - \frac{4}{3} \hat{n} \times \vec{a}_1 \cdot \vec{S}_1 \vec{a}_2 \cdot \vec{V}_2 - \frac{8}{3} \hat{n} \times \vec{a}_1 \cdot \vec{S}_1 \vec{V}_2 \cdot \vec{V}_2 + \frac{8}{3} \hat{n} \times \vec{S}_1 \cdot \vec{V}_1 \vec{V}_2 \cdot \vec{V}_2 - \frac{16}{3} \hat{n} \times \vec{a}_1 \cdot \vec{S}_1 \vec{V}_2 \cdot \vec{V}_2 \right) m_2^2 + \\ & \frac{1}{r^2} G^2 \left( 4 \hat{n} \times \vec{S}_1 \cdot \vec{V}_1 (\hat{n} \cdot \vec{V}_2)^3 - 4 \hat{n} \times \vec{a}_1 \cdot \vec{S}_1 (\hat{n} \cdot \vec{V}_2)^3 - 3 \vec{S}_1 \times \vec{V}_1 \cdot \vec{V}_2 (\hat{n} \cdot \vec{V}_2)^2 + \frac{4}{3} \vec{a}_1 \times \vec{S}_1 \cdot \vec{V}_1 (\hat{n} \cdot \vec{V}_2)^2 + \right. \\ & \quad 3 \vec{a}_1 \times \vec{S}_1 \cdot \vec{V}_2 (\hat{n} \cdot \vec{V}_2)^2 - \frac{8}{3} \vec{a}_2 \times \vec{S}_1 \cdot \vec{V}_1 (\hat{n} \cdot \vec{V}_2)^2 + \frac{16}{3} \hat{n} \times \vec{S}_1 \cdot \vec{V}_1 \hat{n} \cdot \vec{a}_1 (\hat{n} \cdot \vec{V}_2)^2 + \frac{32}{3} \hat{n} \times \vec{S}_1 \cdot \vec{V}_1 \hat{n} \cdot \vec{a}_2 (\hat{n} \cdot \vec{V}_2)^2 + \\ & \quad \frac{32}{3} \hat{n} \times \vec{S}_1 \cdot \vec{V}_1 \hat{n} \cdot \vec{V}_1 (\hat{n} \cdot \vec{V}_2)^2 - \frac{32}{3} \hat{n} \times \vec{a}_1 \cdot \vec{S}_1 \hat{n} \cdot \vec{V}_1 (\hat{n} \cdot \vec{V}_2)^2 - \frac{8}{3} \vec{S}_1 \times \vec{V}_1 \cdot \vec{V}_2 \hat{n} \cdot \vec{a}_1 \hat{n} \cdot \vec{V}_2 - \\ & \quad \frac{16}{3} \vec{S}_1 \times \vec{V}_1 \cdot \vec{V}_2 \hat{n} \cdot \vec{a}_2 \hat{n} \cdot \vec{V}_2 - \frac{16}{3} \vec{S}_1 \times \vec{V}_1 \cdot \vec{V}_2 \hat{n} \cdot \vec{V}_1 \hat{n} \cdot \vec{V}_2 + \frac{16}{3} \vec{a}_1 \times \vec{S}_1 \cdot \vec{V}_2 \hat{n} \cdot \vec{V}_1 \hat{n} \cdot \vec{V}_2 + \\ & \quad \frac{4}{3} \vec{a}_2 \times \vec{S}_1 \cdot \vec{V}_1 \hat{n} \cdot \vec{V}_1 \hat{n} \cdot \vec{V}_2 - \frac{16}{3} \hat{n} \times \vec{S}_1 \cdot \vec{V}_1 \hat{n} \cdot \vec{a}_2 \hat{n} \cdot \vec{V}_1 \hat{n} \cdot \vec{V}_2 - \frac{8}{3} \hat{n} \times \vec{S}_1 \cdot \vec{V}_1 \vec{a}_1 \cdot \vec{V}_2 \hat{n} \cdot \vec{V}_2 + \\ & \quad \frac{4}{3} \hat{n} \times \vec{S}_1 \cdot \vec{V}_1 \vec{a}_2 \cdot \vec{V}_1 \hat{n} \cdot \vec{V}_2 - \frac{4}{3} \hat{n} \times \vec{S}_1 \cdot \vec{V}_1 \vec{a}_2 \cdot \vec{V}_2 \hat{n} \cdot \vec{V}_2 - \frac{16}{3} \hat{n} \times \vec{S}_1 \cdot \vec{V}_1 \vec{V}_1 \cdot \vec{V}_2 \hat{n} \cdot \vec{V}_2 + \frac{16}{3} \hat{n} \times \vec{a}_1 \cdot \vec{S}_1 \vec{V}_1 \cdot \vec{V}_2 \hat{n} \cdot \vec{V}_2 - \\ & \quad 6 \hat{n} \times \vec{S}_1 \cdot \vec{V}_1 \vec{V}_2 \cdot \vec{V}_2 \hat{n} \cdot \vec{V}_2 + 6 \hat{n} \times \vec{a}_1 \cdot \vec{S}_1 \vec{V}_2 \cdot \vec{V}_2 \hat{n} \cdot \vec{V}_2 + \frac{4}{3} \vec{S}_1 \times \vec{V}_1 \cdot \vec{V}_2 \hat{n} \cdot \vec{a}_2 \hat{n} \cdot \vec{V}_1 + \frac{4}{3} \vec{S}_1 \times \vec{V}_1 \cdot \vec{V}_2 \vec{a}_1 \cdot \vec{V}_2 - \\ & \quad \frac{2}{3} \vec{S}_1 \times \vec{V}_1 \cdot \vec{V}_2 \vec{a}_2 \cdot \vec{V}_1 + \frac{2}{3} \vec{S}_1 \times \vec{V}_1 \cdot \vec{V}_2 \vec{a}_2 \cdot \vec{V}_2 - \frac{8}{3} \hat{n} \times \vec{S}_1 \cdot \vec{V}_1 \hat{n} \cdot \vec{V}_1 \vec{a}_2 \cdot \vec{V}_2 + \frac{8}{3} \frac{1}{\vec{S}_1 \times \vec{V}_1} \cdot \vec{V}_2 \vec{V}_1 \cdot \vec{V}_2 - \\ & \quad \frac{8}{3} \vec{a}_1 \times \vec{S}_1 \cdot \vec{V}_2 \vec{V}_1 \cdot \vec{V}_2 - \frac{2}{3} \vec{a}_2 \times \vec{S}_1 \cdot \vec{V}_1 \vec{V}_1 \cdot \vec{V}_2 + \frac{4}{3} \hat{n} \times \vec{S}_1 \cdot \vec{V}_1 \hat{n} \cdot \vec{a}_2 \vec{V}_1 \cdot \vec{V}_2 + 3 \vec{S}_1 \times \vec{V}_1 \cdot \vec{V}_2 \vec{V}_2 \cdot \vec{V}_2 - \\ & \quad \frac{8}{3} \vec{a}_1 \times \vec{S}_1 \cdot \vec{V}_1 \vec{V}_2 \cdot \vec{V}_2 - 3 \vec{a}_1 \times \vec{S}_1 \cdot \vec{V}_2 \vec{V}_2 \cdot \vec{V}_2 + \frac{10}{3} \vec{a}_2 \times \vec{S}_1 \cdot \vec{V}_1 \vec{V}_2 \cdot \vec{V}_2 - \frac{16}{3} \hat{n} \times \vec{S}_1 \cdot \vec{V}_1 \hat{n} \cdot \vec{a}_1 \vec{V}_2 \cdot \vec{V}_2 - \\ & \quad \left. \frac{20}{3} \hat{n} \times \vec{S}_1 \cdot \vec{V}_1 \hat{n} \cdot \vec{a}_2 \vec{V}_2 \cdot \vec{V}_2 - \frac{32}{3} \hat{n} \times \vec{S}_1 \cdot \vec{V}_1 \hat{n} \cdot \vec{V}_1 \vec{V}_2 \cdot \vec{V}_2 + \frac{32}{3} \hat{n} \times \vec{a}_1 \cdot \vec{S}_1 \hat{n} \cdot \vec{V}_1 \vec{V}_2 \cdot \vec{V}_2 \right) m_2^2 + \\ & \frac{1}{r^3} G^2 \left( 8 \hat{n} \times \vec{S}_1 \cdot \vec{V}_1 (\hat{n} \cdot \vec{V}_2)^4 - \frac{16}{3} \vec{S}_1 \times \vec{V}_1 \cdot \vec{V}_2 (\hat{n} \cdot \vec{V}_2)^3 - 24 \hat{n} \times \vec{S}_1 \cdot \vec{V}_1 \hat{n} \cdot \vec{V}_1 (\hat{n} \cdot \vec{V}_2)^3 - \right. \\ & \quad \left. 32 \hat{n} \times \vec{S}_1 \cdot \vec{V}_1 (\hat{n} \cdot \vec{V}_1)^2 (\hat{n} \cdot \vec{V}_2)^2 + 12 \vec{S}_1 \times \vec{V}_1 \cdot \vec{V}_2 \hat{n} \cdot \vec{V}_1 (\hat{n} \cdot \vec{V}_2)^2 + \frac{16}{3} \hat{n} \times \vec{S}_1 \cdot \vec{V}_1 \vec{V}_1 \cdot \vec{V}_1 (\hat{n} \cdot \vec{V}_2)^2 + \right. \end{aligned}$$

$$\begin{aligned}
& 12 \hat{n} \times \vec{S}_1 \cdot \vec{v}_1 \vec{v}_1 \cdot \vec{v}_2 (\hat{n} \cdot \vec{v}_2)^2 - 12 \hat{n} \times \vec{S}_1 \cdot \vec{v}_1 \vec{v}_2 \cdot \vec{v}_2 (\hat{n} \cdot \vec{v}_2)^2 + \frac{32}{3} \vec{S}_1 \times \vec{v}_1 \cdot \vec{v}_2 (\hat{n} \cdot \vec{v}_1)^2 \hat{n} \cdot \vec{v}_2 - \\
& \frac{8}{3} \vec{S}_1 \times \vec{v}_1 \cdot \vec{v}_2 \vec{v}_1 \cdot \vec{v}_1 \hat{n} \cdot \vec{v}_2 - 6 \vec{S}_1 \times \vec{v}_1 \cdot \vec{v}_2 \vec{v}_1 \cdot \vec{v}_2 \hat{n} \cdot \vec{v}_2 + \frac{64}{3} \hat{n} \times \vec{S}_1 \cdot \vec{v}_1 \hat{n} \cdot \vec{v}_1 \vec{v}_1 \cdot \vec{v}_2 \hat{n} \cdot \vec{v}_2 + \\
& 6 \vec{S}_1 \times \vec{v}_1 \cdot \vec{v}_2 \vec{v}_2 \cdot \vec{v}_2 \hat{n} \cdot \vec{v}_2 + 24 \hat{n} \times \vec{S}_1 \cdot \vec{v}_1 \hat{n} \cdot \vec{v}_1 \vec{v}_2 \cdot \vec{v}_2 \hat{n} \cdot \vec{v}_2 - \frac{8}{3} \hat{n} \times \vec{S}_1 \cdot \vec{v}_1 (\vec{v}_1 \cdot \vec{v}_2)^2 + \\
& 2 \hat{n} \times \vec{S}_1 \cdot \vec{v}_1 (\vec{v}_2 \cdot \vec{v}_2)^2 - \frac{16}{3} \vec{S}_1 \times \vec{v}_1 \cdot \vec{v}_2 \hat{n} \cdot \vec{v}_1 \vec{v}_1 \cdot \vec{v}_2 + \frac{64}{3} \hat{n} \times \vec{S}_1 \cdot \vec{v}_1 (\hat{n} \cdot \vec{v}_1)^2 \vec{v}_2 \cdot \vec{v}_2 - \\
& 6 \vec{S}_1 \times \vec{v}_1 \cdot \vec{v}_2 \hat{n} \cdot \vec{v}_1 \vec{v}_2 \cdot \vec{v}_2 - \frac{16}{3} \hat{n} \times \vec{S}_1 \cdot \vec{v}_1 \vec{v}_1 \cdot \vec{v}_1 \vec{v}_2 \cdot \vec{v}_2 - 6 \hat{n} \times \vec{S}_1 \cdot \vec{v}_1 \vec{v}_1 \cdot \vec{v}_2 \vec{v}_2 \cdot \vec{v}_2 \Big) m_2^2 \Big\}
\end{aligned}$$

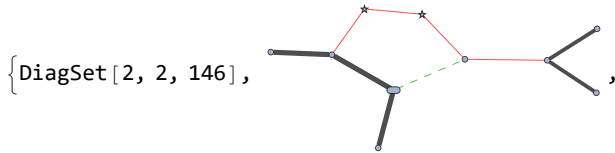

$$\begin{aligned}
& \frac{1}{r} \left( -\frac{3}{16} \hat{n} \times \vec{S}_1 \cdot \vec{v}_1 (\hat{n} \cdot \vec{a}_1)^2 - \frac{1}{3} \vec{S}_1 \times \vec{v}_1 \cdot \vec{v}_2 \hat{n} \cdot \vec{a}_1 - \frac{1}{6} \vec{S}_1 \times \vec{a}_1 \cdot \vec{v}_2 \hat{n} \cdot \vec{a}_1 + \frac{1}{8} \vec{S}_1 \times \vec{v}_1 \cdot \vec{a}_1 \hat{n} \cdot \vec{a}_1 - \right. \\
& \frac{5}{24} \vec{S}_1 \times \vec{v}_1 \cdot \vec{a}_2 \hat{n} \cdot \vec{a}_1 + \frac{5}{12} \hat{n} \times \vec{S}_1 \cdot \vec{v}_1 \hat{n} \cdot \vec{a}_2 \hat{n} \cdot \vec{a}_1 - \frac{1}{4} \hat{n} \times \vec{S}_1 \cdot \vec{v}_1 \hat{n} \cdot \vec{v}_1 \hat{n} \cdot \vec{a}_1 - \frac{1}{8} \hat{n} \times \vec{S}_1 \cdot \vec{a}_1 \hat{n} \cdot \vec{v}_1 \hat{n} \cdot \vec{a}_1 + \\
& \frac{2}{3} \hat{n} \times \vec{S}_1 \cdot \vec{v}_1 \hat{n} \cdot \vec{v}_2 \hat{n} \cdot \vec{a}_1 + \frac{1}{3} \hat{n} \times \vec{S}_1 \cdot \vec{a}_1 \hat{n} \cdot \vec{v}_2 \hat{n} \cdot \vec{a}_1 - \frac{3}{8} \hat{n} \times \vec{S}_1 \cdot \vec{a}_1 (\hat{n} \cdot \vec{v}_1)^2 - \frac{1}{16} \hat{n} \times \vec{S}_1 \cdot \vec{v}_1 (\hat{n} \cdot \vec{v}_1)^2 + \\
& \frac{5}{16} \hat{n} \times \vec{S}_1 \cdot \vec{a}_1 (\hat{n} \cdot \vec{v}_1)^2 - \frac{1}{3} \hat{n} \times \vec{S}_1 \cdot \vec{a}_1 (\hat{n} \cdot \vec{v}_2)^2 + \frac{1}{6} \hat{n} \times \vec{S}_1 \cdot \vec{a}_1 (\hat{n} \cdot \vec{v}_2)^2 + \frac{1}{12} \vec{S}_1 \times \vec{v}_1 \cdot \vec{v}_2 \hat{n} \cdot \vec{a}_1 + \\
& \frac{1}{4} \vec{S}_1 \times \vec{a}_1 \cdot \vec{v}_2 \hat{n} \cdot \vec{a}_2 + \frac{1}{6} \vec{S}_1 \times \vec{v}_1 \cdot \vec{a}_1 \hat{n} \cdot \vec{a}_2 - \frac{1}{2} \vec{S}_1 \times \vec{a}_1 \cdot \vec{v}_2 \hat{n} \cdot \vec{v}_1 - \frac{1}{4} \vec{S}_1 \times \vec{v}_1 \cdot \vec{a}_1 \hat{n} \cdot \vec{v}_1 + \frac{1}{6} \vec{S}_1 \times \vec{v}_1 \cdot \vec{a}_2 \hat{n} \cdot \vec{v}_1 + \\
& \frac{1}{12} \vec{S}_1 \times \vec{v}_1 \cdot \vec{v}_2 \hat{n} \cdot \vec{v}_1 + \frac{1}{4} \vec{S}_1 \times \vec{a}_1 \cdot \vec{v}_2 \hat{n} \cdot \vec{v}_1 - \frac{3}{8} \vec{S}_1 \times \vec{a}_1 \cdot \vec{a}_2 \hat{n} \cdot \vec{v}_1 + \frac{1}{4} \vec{S}_1 \times \vec{v}_1 \cdot \vec{a}_1 \hat{n} \cdot \vec{v}_1 + \\
& \frac{1}{12} \vec{S}_1 \times \vec{v}_1 \cdot \vec{a}_2 \hat{n} \cdot \vec{v}_1 + \frac{1}{8} \hat{n} \times \vec{S}_1 \cdot \vec{v}_1 \hat{n} \cdot \vec{a}_1 \hat{n} \cdot \vec{v}_1 - \frac{1}{6} \hat{n} \times \vec{S}_1 \cdot \vec{v}_1 \hat{n} \cdot \vec{a}_2 \hat{n} \cdot \vec{v}_1 - \frac{1}{3} \hat{n} \times \vec{S}_1 \cdot \vec{v}_1 \hat{n} \cdot \vec{a}_2 \hat{n} \cdot \vec{v}_1 + \\
& \frac{3}{4} \hat{n} \times \vec{S}_1 \cdot \vec{a}_1 \hat{n} \cdot \vec{a}_2 \hat{n} \cdot \vec{v}_1 + \frac{1}{3} \vec{S}_1 \times \vec{a}_1 \cdot \vec{v}_2 \hat{n} \cdot \vec{v}_2 + \frac{1}{6} \vec{S}_1 \times \vec{v}_1 \cdot \vec{a}_1 \hat{n} \cdot \vec{v}_2 - \frac{1}{6} \vec{S}_1 \times \vec{a}_1 \cdot \vec{v}_2 \hat{n} \cdot \vec{v}_2 + \\
& \frac{1}{4} \vec{S}_1 \times \vec{a}_1 \cdot \vec{a}_2 \hat{n} \cdot \vec{v}_2 - \frac{1}{6} \vec{S}_1 \times \vec{v}_1 \cdot \vec{a}_1 \hat{n} \cdot \vec{v}_2 - \frac{1}{6} \hat{n} \times \vec{S}_1 \cdot \vec{v}_1 \hat{n} \cdot \vec{a}_1 \hat{n} \cdot \vec{v}_2 - \frac{1}{2} \hat{n} \times \vec{S}_1 \cdot \vec{a}_1 \hat{n} \cdot \vec{a}_2 \hat{n} \cdot \vec{v}_2 + \\
& \hat{n} \times \vec{S}_1 \cdot \vec{a}_1 \hat{n} \cdot \vec{v}_1 \hat{n} \cdot \vec{v}_2 - \frac{1}{6} \hat{n} \times \vec{S}_1 \cdot \vec{v}_1 \hat{n} \cdot \vec{v}_1 \hat{n} \cdot \vec{v}_2 - \frac{1}{2} \hat{n} \times \vec{S}_1 \cdot \vec{a}_1 \hat{n} \cdot \vec{v}_1 \hat{n} \cdot \vec{v}_2 + \frac{1}{12} \hat{n} \times \vec{S}_1 \cdot \vec{v}_1 \vec{a}_1 \cdot \vec{v}_2 - \\
& \frac{3}{16} \hat{n} \times \vec{S}_1 \cdot \vec{v}_1 \vec{a}_1 \cdot \vec{a}_1 - \frac{5}{24} \hat{n} \times \vec{S}_1 \cdot \vec{v}_1 \vec{a}_1 \cdot \vec{a}_2 - \frac{1}{3} \hat{n} \times \vec{S}_1 \cdot \vec{v}_1 \vec{a}_1 \cdot \vec{v}_2 - \frac{1}{6} \hat{n} \times \vec{S}_1 \cdot \vec{a}_1 \vec{a}_1 \cdot \vec{v}_2 + \frac{1}{8} \hat{n} \times \vec{S}_1 \cdot \vec{v}_1 \vec{v}_1 \cdot \vec{a}_1 + \\
& \frac{1}{12} \hat{n} \times \vec{S}_1 \cdot \vec{v}_1 \vec{v}_1 \cdot \vec{a}_2 - \hat{n} \times \vec{S}_1 \cdot \vec{v}_1 \vec{v}_1 \cdot \vec{a}_1 - \frac{1}{2} \hat{n} \times \vec{S}_1 \cdot \vec{a}_1 \vec{v}_1 \cdot \vec{a}_1 + \frac{1}{6} \hat{n} \times \vec{S}_1 \cdot \vec{v}_1 \vec{v}_1 \cdot \vec{a}_2 - \frac{3}{8} \hat{n} \times \vec{S}_1 \cdot \vec{a}_1 \vec{v}_1 \cdot \vec{a}_2 - \\
& \frac{3}{8} \hat{n} \times \vec{S}_1 \cdot \vec{a}_1 \vec{v}_1 \cdot \vec{v}_1 + \frac{5}{16} \hat{n} \times \vec{S}_1 \cdot \vec{v}_1 \vec{v}_1 \cdot \vec{v}_1 - \frac{1}{16} \hat{n} \times \vec{S}_1 \cdot \vec{a}_1 \vec{v}_1 \cdot \vec{v}_1 - \frac{1}{2} \hat{n} \times \vec{S}_1 \cdot \vec{a}_1 \vec{v}_1 \cdot \vec{v}_2 + \frac{1}{12} \hat{n} \times \vec{S}_1 \cdot \vec{v}_1 \vec{v}_1 \cdot \vec{v}_2 + \\
& \frac{1}{4} \hat{n} \times \vec{S}_1 \cdot \vec{a}_1 \vec{v}_1 \cdot \vec{v}_2 + \frac{1}{4} \hat{n} \times \vec{S}_1 \cdot \vec{a}_1 \vec{v}_2 \cdot \vec{a}_2 + \frac{1}{6} \hat{n} \times \vec{S}_1 \cdot \vec{a}_1 \vec{v}_2 \cdot \vec{v}_2 - \frac{1}{12} \hat{n} \times \vec{S}_1 \cdot \vec{a}_1 \vec{v}_2 \cdot \vec{v}_2 \Big) m_1 m_2 G^2 + \frac{1}{r^2} \\
& \left( \frac{1}{6} \hat{n} \times \vec{S}_1 \cdot \vec{v}_1 (\hat{n} \cdot \vec{v}_1)^3 + \frac{7}{12} \hat{n} \times \vec{S}_1 \cdot \vec{a}_1 (\hat{n} \cdot \vec{v}_1)^3 - \frac{1}{12} \vec{S}_1 \times \vec{v}_1 \cdot \vec{v}_2 (\hat{n} \cdot \vec{v}_1)^2 + \frac{17}{24} \vec{S}_1 \times \vec{a}_1 \cdot \vec{v}_2 (\hat{n} \cdot \vec{v}_1)^2 + \right. \\
& \frac{5}{16} \vec{S}_1 \times \vec{v}_1 \cdot \vec{a}_1 (\hat{n} \cdot \vec{v}_1)^2 - \frac{7}{48} \vec{S}_1 \times \vec{v}_1 \cdot \vec{a}_2 (\hat{n} \cdot \vec{v}_1)^2 + \frac{1}{2} \hat{n} \times \vec{S}_1 \cdot \vec{v}_1 \hat{n} \cdot \vec{a}_1 (\hat{n} \cdot \vec{v}_1)^2 + \frac{7}{12} \hat{n} \times \vec{S}_1 \cdot \vec{v}_1 \hat{n} \cdot \vec{a}_2 (\hat{n} \cdot \vec{v}_1)^2 + \\
& \frac{1}{3} \hat{n} \times \vec{S}_1 \cdot \vec{v}_1 \hat{n} \cdot \vec{v}_2 (\hat{n} \cdot \vec{v}_1)^2 - \frac{17}{6} \hat{n} \times \vec{S}_1 \cdot \vec{a}_1 \hat{n} \cdot \vec{v}_2 (\hat{n} \cdot \vec{v}_1)^2 - \frac{4}{3} \hat{n} \times \vec{S}_1 \cdot \vec{v}_1 (\hat{n} \cdot \vec{v}_2)^2 \hat{n} \cdot \vec{v}_1 + \\
& \left. 3 \hat{n} \times \vec{S}_1 \cdot \vec{a}_1 (\hat{n} \cdot \vec{v}_2)^2 \hat{n} \cdot \vec{v}_1 + \frac{1}{4} \vec{S}_1 \times \vec{v}_1 \cdot \vec{v}_2 \hat{n} \cdot \vec{a}_1 \hat{n} \cdot \vec{v}_1 + \frac{1}{2} \vec{S}_1 \times \vec{v}_1 \cdot \vec{v}_2 \hat{n} \cdot \vec{a}_2 \hat{n} \cdot \vec{v}_1 + \frac{2}{3} \vec{S}_1 \times \vec{v}_1 \cdot \vec{v}_2 \hat{n} \cdot \vec{v}_2 \hat{n} \cdot \vec{v}_1 - \right.
\end{aligned}$$



$$\begin{aligned}
& \frac{3}{2} \vec{S}_1 \times \vec{a}_1 \cdot \vec{v}_2 \hat{n} \cdot \vec{v}_2 \hat{n} \cdot \vec{v}_1 - \frac{7}{6} \vec{S}_1 \times \vec{v}_1 \cdot \vec{a}_1 \hat{n} \cdot \vec{v}_2 \hat{n} \cdot \vec{v}_1 + \frac{1}{2} \vec{S}_1 \times \vec{v}_1 \cdot \vec{a}_2 \hat{n} \cdot \vec{v}_2 \hat{n} \cdot \vec{v}_1 - \hat{n} \times \vec{S}_1 \cdot \vec{v}_1 \hat{n} \cdot \vec{a}_1 \hat{n} \cdot \vec{v}_2 \hat{n} \cdot \vec{v}_1 - \\
& 2 \hat{n} \times \vec{S}_1 \cdot \vec{v}_1 \hat{n} \cdot \vec{a}_2 \hat{n} \cdot \vec{v}_2 \hat{n} \cdot \vec{v}_1 + \frac{1}{4} \hat{n} \times \vec{S}_1 \cdot \vec{v}_1 \vec{a}_1 \cdot \vec{v}_2 \hat{n} \cdot \vec{v}_1 + \frac{13}{8} \hat{n} \times \vec{S}_1 \cdot \vec{v}_1 \vec{v}_1 \cdot \vec{a}_1 \hat{n} \cdot \vec{v}_1 - \\
& \frac{7}{24} \hat{n} \times \vec{S}_1 \cdot \vec{v}_1 \vec{v}_1 \cdot \vec{a}_2 \hat{n} \cdot \vec{v}_1 - \frac{1}{2} \hat{n} \times \vec{S}_1 \cdot \vec{v}_1 \vec{v}_1 \cdot \vec{v}_1 \hat{n} \cdot \vec{v}_1 + \frac{1}{2} \hat{n} \times \vec{S}_1 \cdot \vec{a}_1 \vec{v}_1 \cdot \vec{v}_1 \hat{n} \cdot \vec{v}_1 - \frac{1}{6} \hat{n} \times \vec{S}_1 \cdot \vec{v}_1 \vec{v}_1 \cdot \vec{v}_2 \hat{n} \cdot \vec{v}_1 + \\
& \frac{17}{12} \hat{n} \times \vec{S}_1 \cdot \vec{a}_1 \vec{v}_1 \cdot \vec{v}_2 \hat{n} \cdot \vec{v}_1 + \frac{1}{2} \hat{n} \times \vec{S}_1 \cdot \vec{v}_1 \vec{v}_2 \cdot \vec{a}_2 \hat{n} \cdot \vec{v}_1 + \frac{1}{3} \hat{n} \times \vec{S}_1 \cdot \vec{v}_1 \vec{v}_2 \cdot \vec{v}_2 \hat{n} \cdot \vec{v}_1 - \frac{3}{4} \hat{n} \times \vec{S}_1 \cdot \vec{a}_1 \vec{v}_2 \cdot \vec{v}_2 \hat{n} \cdot \vec{v}_1 - \\
& \frac{2}{3} \hat{n} \times \vec{S}_1 \cdot \vec{a}_1 (\hat{n} \cdot \vec{v}_2)^3 + \frac{1}{2} \vec{S}_1 \times \vec{a}_1 \cdot \vec{v}_2 (\hat{n} \cdot \vec{v}_2)^2 + \frac{1}{3} \vec{S}_1 \times \vec{v}_1 \cdot \vec{a}_1 (\hat{n} \cdot \vec{v}_2)^2 + \frac{5}{3} \hat{n} \times \vec{S}_1 \cdot \vec{v}_1 \hat{n} \cdot \vec{a}_1 (\hat{n} \cdot \vec{v}_2)^2 - \\
& \frac{5}{6} \vec{S}_1 \times \vec{v}_1 \cdot \vec{v}_2 \hat{n} \cdot \vec{a}_1 \hat{n} \cdot \vec{v}_2 + \frac{5}{12} \vec{S}_1 \times \vec{v}_1 \cdot \vec{v}_2 \vec{a}_1 \cdot \vec{v}_2 - \frac{5}{6} \hat{n} \times \vec{S}_1 \cdot \vec{v}_1 \hat{n} \cdot \vec{v}_2 \vec{a}_1 \cdot \vec{v}_2 + \vec{S}_1 \times \vec{v}_1 \cdot \vec{v}_2 \vec{v}_1 \cdot \vec{a}_1 - \\
& 2 \hat{n} \times \vec{S}_1 \cdot \vec{v}_1 \hat{n} \cdot \vec{v}_2 \vec{v}_1 \cdot \vec{a}_1 - \frac{1}{4} \vec{S}_1 \times \vec{v}_1 \cdot \vec{v}_2 \vec{v}_1 \cdot \vec{a}_2 + \frac{1}{2} \hat{n} \times \vec{S}_1 \cdot \vec{v}_1 \hat{n} \cdot \vec{v}_2 \vec{v}_1 \cdot \vec{a}_2 - \frac{13}{12} \frac{1}{\vec{S}_1 \times \vec{v}_1 \cdot \vec{v}_2 \vec{v}_1 \cdot \vec{v}_1} + \\
& \frac{5}{24} \vec{S}_1 \times \vec{a}_1 \cdot \vec{v}_2 \vec{v}_1 \cdot \vec{v}_1 + \frac{11}{16} \vec{S}_1 \times \vec{v}_1 \cdot \vec{a}_1 \vec{v}_1 \cdot \vec{v}_1 - \frac{37}{48} \vec{S}_1 \times \vec{v}_1 \cdot \vec{a}_2 \vec{v}_1 \cdot \vec{v}_1 - \frac{7}{8} \hat{n} \times \vec{S}_1 \cdot \vec{v}_1 \hat{n} \cdot \vec{a}_1 \vec{v}_1 \cdot \vec{v}_1 + \\
& \frac{37}{24} \hat{n} \times \vec{S}_1 \cdot \vec{v}_1 \hat{n} \cdot \vec{a}_2 \vec{v}_1 \cdot \vec{v}_1 + \frac{13}{6} \hat{n} \times \vec{S}_1 \cdot \vec{v}_1 \hat{n} \cdot \vec{v}_2 \vec{v}_1 \cdot \vec{v}_1 - \frac{5}{12} \hat{n} \times \vec{S}_1 \cdot \vec{a}_1 \hat{n} \cdot \vec{v}_2 \vec{v}_1 \cdot \vec{v}_1 - \frac{1}{3} \frac{1}{\vec{S}_1 \times \vec{v}_1 \cdot \vec{v}_2 \vec{v}_1 \cdot \vec{v}_2} + \\
& \frac{3}{4} \vec{S}_1 \times \vec{a}_1 \cdot \vec{v}_2 \vec{v}_1 \cdot \vec{v}_2 + \frac{7}{12} \vec{S}_1 \times \vec{v}_1 \cdot \vec{a}_1 \vec{v}_1 \cdot \vec{v}_2 - \frac{1}{4} \vec{S}_1 \times \vec{v}_1 \cdot \vec{a}_2 \vec{v}_1 \cdot \vec{v}_2 + \frac{1}{4} \hat{n} \times \vec{S}_1 \cdot \vec{v}_1 \hat{n} \cdot \vec{a}_1 \vec{v}_1 \cdot \vec{v}_2 + \\
& \frac{1}{2} \hat{n} \times \vec{S}_1 \cdot \vec{v}_1 \hat{n} \cdot \vec{a}_2 \vec{v}_1 \cdot \vec{v}_2 + \frac{2}{3} \hat{n} \times \vec{S}_1 \cdot \vec{v}_1 \hat{n} \cdot \vec{v}_2 \vec{v}_1 \cdot \vec{v}_2 - \frac{3}{2} \hat{n} \times \vec{S}_1 \cdot \vec{a}_1 \hat{n} \cdot \vec{v}_2 \vec{v}_1 \cdot \vec{v}_2 - \frac{1}{4} \vec{S}_1 \times \vec{a}_1 \cdot \vec{v}_2 \vec{v}_2 \cdot \vec{v}_2 - \\
& \frac{1}{6} \vec{S}_1 \times \vec{v}_1 \cdot \vec{a}_1 \vec{v}_2 \cdot \vec{v}_2 - \frac{5}{12} \hat{n} \times \vec{S}_1 \cdot \vec{v}_1 \hat{n} \cdot \vec{a}_1 \vec{v}_2 \cdot \vec{v}_2 + \frac{1}{2} \hat{n} \times \vec{S}_1 \cdot \vec{a}_1 \hat{n} \cdot \vec{v}_2 \vec{v}_2 \cdot \vec{v}_2 \Big) m_1 m_2 G^2 + \frac{1}{r^3} \\
& \left( -\frac{9}{32} \hat{n} \times \vec{S}_1 \cdot \vec{v}_1 (\hat{n} \cdot \vec{v}_1)^4 + \frac{1}{6} \vec{S}_1 \times \vec{v}_1 \cdot \vec{v}_2 (\hat{n} \cdot \vec{v}_1)^3 - \hat{n} \times \vec{S}_1 \cdot \vec{v}_1 \hat{n} \cdot \vec{v}_2 (\hat{n} \cdot \vec{v}_1)^3 + \frac{7}{2} \hat{n} \times \vec{S}_1 \cdot \vec{v}_1 (\hat{n} \cdot \vec{v}_2)^2 (\hat{n} \cdot \vec{v}_1)^2 - \right. \\
& \frac{7}{6} \vec{S}_1 \times \vec{v}_1 \cdot \vec{v}_2 \hat{n} \cdot \vec{v}_2 (\hat{n} \cdot \vec{v}_1)^2 + \frac{15}{16} \hat{n} \times \vec{S}_1 \cdot \vec{v}_1 \vec{v}_1 \cdot \vec{v}_1 (\hat{n} \cdot \vec{v}_1)^2 + \frac{1}{2} \hat{n} \times \vec{S}_1 \cdot \vec{v}_1 \vec{v}_1 \cdot \vec{v}_2 (\hat{n} \cdot \vec{v}_1)^2 - \\
& \frac{7}{12} \hat{n} \times \vec{S}_1 \cdot \vec{v}_1 \vec{v}_2 \cdot \vec{v}_2 (\hat{n} \cdot \vec{v}_1)^2 - 4 \hat{n} \times \vec{S}_1 \cdot \vec{v}_1 (\hat{n} \cdot \vec{v}_2)^3 \hat{n} \cdot \vec{v}_1 + 2 \vec{S}_1 \times \vec{v}_1 \cdot \vec{v}_2 (\hat{n} \cdot \vec{v}_2)^2 \hat{n} \cdot \vec{v}_1 + \vec{S}_1 \times \vec{v}_1 \cdot \vec{v}_2 \vec{v}_1 \cdot \vec{v}_1 \hat{n} \cdot \vec{v}_1 - \\
& 4 \hat{n} \times \vec{S}_1 \cdot \vec{v}_1 \hat{n} \cdot \vec{v}_2 \vec{v}_1 \cdot \vec{v}_1 \hat{n} \cdot \vec{v}_1 + \frac{7}{12} \vec{S}_1 \times \vec{v}_1 \cdot \vec{v}_2 \vec{v}_1 \cdot \vec{v}_2 \hat{n} \cdot \vec{v}_1 - \frac{7}{3} \hat{n} \times \vec{S}_1 \cdot \vec{v}_1 \hat{n} \cdot \vec{v}_2 \vec{v}_1 \cdot \vec{v}_2 \hat{n} \cdot \vec{v}_1 - \\
& \frac{1}{2} \vec{S}_1 \times \vec{v}_1 \cdot \vec{v}_2 \vec{v}_2 \cdot \vec{v}_2 \hat{n} \cdot \vec{v}_1 + 2 \hat{n} \times \vec{S}_1 \cdot \vec{v}_1 \hat{n} \cdot \vec{v}_2 \vec{v}_2 \cdot \vec{v}_2 \hat{n} \cdot \vec{v}_1 + \frac{3}{32} \hat{n} \times \vec{S}_1 \cdot \vec{v}_1 (\vec{v}_1 \cdot \vec{v}_1)^2 + \frac{7}{24} \hat{n} \times \vec{S}_1 \cdot \vec{v}_1 (\vec{v}_1 \cdot \vec{v}_2)^2 + \\
& \frac{37}{6} \hat{n} \times \vec{S}_1 \cdot \vec{v}_1 (\hat{n} \cdot \vec{v}_2)^2 \vec{v}_1 \cdot \vec{v}_1 - \frac{37}{12} \vec{S}_1 \times \vec{v}_1 \cdot \vec{v}_2 \hat{n} \cdot \vec{v}_2 \vec{v}_1 \cdot \vec{v}_1 + 2 \hat{n} \times \vec{S}_1 \cdot \vec{v}_1 (\hat{n} \cdot \vec{v}_2)^2 \vec{v}_1 \cdot \vec{v}_2 - \vec{S}_1 \times \vec{v}_1 \cdot \vec{v}_2 \hat{n} \cdot \vec{v}_2 \vec{v}_1 \cdot \vec{v}_2 + \\
& \left. \hat{n} \times \vec{S}_1 \cdot \vec{v}_1 \vec{v}_1 \cdot \vec{v}_1 \vec{v}_1 \cdot \vec{v}_2 - \frac{37}{24} \hat{n} \times \vec{S}_1 \cdot \vec{v}_1 \vec{v}_1 \cdot \vec{v}_1 \vec{v}_2 \cdot \vec{v}_2 - \frac{1}{2} \hat{n} \times \vec{S}_1 \cdot \vec{v}_1 \vec{v}_1 \cdot \vec{v}_2 \vec{v}_2 \cdot \vec{v}_2 \right) m_1 m_2 G^2 + \\
& r m_1 m_2 \left( -\frac{1}{12} \log \left( \frac{r}{R_\theta} \right) \hat{n} \times \vec{S}_1 \cdot \vec{a}_1 + \frac{\hat{n} \times \vec{S}_1 \cdot \vec{a}_1}{24 \epsilon_d} + \frac{17}{144} \hat{n} \times \vec{S}_1 \cdot \frac{1}{\vec{a}_1} \right) G^2 + \\
& m_1 m_2 \left( \frac{1}{6} \log \left( \frac{r}{R_\theta} \right) \frac{1}{\vec{S}_1 \times \vec{a}_1 \cdot \vec{v}_2} - \frac{17}{72} \frac{1}{\vec{S}_1 \times \vec{a}_1 \cdot \vec{v}_2} + \frac{17}{72} \frac{1}{\vec{S}_1 \times \vec{a}_1 \cdot \vec{a}_2} - \frac{17}{72} \frac{1}{\vec{S}_1 \times \vec{v}_1 \cdot \vec{a}_1} + \frac{17}{144} \frac{2}{\vec{S}_1 \times \vec{a}_1 \cdot \vec{v}_2} - \right. \\
& \frac{17}{144} \vec{S}_1 \times \vec{a}_1 \cdot \vec{a}_2 - \frac{17}{144} \vec{S}_1 \times \vec{a}_1 \cdot \vec{a}_1 + \frac{17}{144} \vec{S}_1 \times \vec{a}_1 \cdot \vec{a}_2 - \frac{1}{12} \hat{n} \times \vec{S}_1 \cdot \vec{v}_1 \hat{n} \cdot \vec{a}_1 - \frac{1}{24} \hat{n} \times \vec{S}_1 \cdot \vec{a}_1 \hat{n} \cdot \vec{a}_1 - \\
& \frac{1}{12} \hat{n} \times \vec{S}_1 \cdot \vec{a}_1 \hat{n} \cdot \vec{a}_2 + \frac{1}{8} \hat{n} \times \vec{S}_1 \cdot \vec{v}_1 \hat{n} \cdot \vec{a}_1 - \frac{1}{8} \hat{n} \times \vec{S}_1 \cdot \vec{a}_1 \hat{n} \cdot \vec{a}_1 - \frac{1}{6} \hat{n} \times \vec{S}_1 \cdot \vec{a}_1 \hat{n} \cdot \vec{a}_2 + \\
& \frac{1}{12} \hat{n} \times \vec{S}_1 \cdot \vec{a}_1 \hat{n} \cdot \vec{a}_2 - \frac{1}{4} \hat{n} \times \vec{S}_1 \cdot \frac{1}{\vec{a}_1} \hat{n} \cdot \vec{v}_1 + \frac{1}{8} \hat{n} \times \vec{S}_1 \cdot \vec{a}_1 \hat{n} \cdot \vec{v}_1 + \frac{1}{6} \hat{n} \times \vec{S}_1 \cdot \frac{1}{\vec{a}_1} \hat{n} \cdot \vec{v}_2 - \frac{1}{12} \hat{n} \times \vec{S}_1 \cdot \vec{a}_1 \hat{n} \cdot \vec{v}_2 - \\
& \frac{1}{6} \frac{1}{\vec{S}_1 \times \vec{a}_1 \cdot \vec{a}_2} \log \left( \frac{r}{R_\theta} \right) + \frac{1}{6} \frac{1}{\vec{S}_1 \times \vec{v}_1 \cdot \vec{a}_1} \log \left( \frac{r}{R_\theta} \right) - \frac{1}{12} \frac{2}{\vec{S}_1 \times \vec{a}_1 \cdot \vec{v}_2} \log \left( \frac{r}{R_\theta} \right) + \frac{1}{12} \vec{S}_1 \times \vec{a}_1 \cdot \vec{a}_2 \log \left( \frac{r}{R_\theta} \right) + \\
& \left. \frac{1}{12} \vec{S}_1 \times \vec{a}_1 \cdot \frac{1}{\vec{a}_1} \log \left( \frac{r}{R_\theta} \right) - \frac{1}{12} \vec{S}_1 \times \vec{a}_1 \cdot \frac{1}{\vec{a}_2} \log \left( \frac{r}{R_\theta} \right) + \frac{1}{\epsilon_d} \left( -\frac{1}{12} \frac{1}{\vec{S}_1 \times \vec{a}_1 \cdot \vec{v}_2} + \frac{1}{12} \frac{1}{\vec{S}_1 \times \vec{a}_1 \cdot \vec{a}_2} - \right. \right.
\end{aligned}$$

$$\left. \left. \left. \frac{1}{12} \vec{S}_1 \times \vec{v}_1 \cdot \vec{a}_1 + \frac{1}{24} \vec{S}_1 \times \vec{a}_1 \cdot \vec{v}_2 - \frac{1}{24} \vec{S}_1 \times \vec{a}_1 \cdot \vec{a}_2 - \frac{1}{24} \vec{S}_1 \times \vec{a}_1 \cdot \vec{a}_1 + \frac{1}{24} \vec{S}_1 \times \vec{a}_1 \cdot \vec{a}_2 \right) \right) \right\} G^2 \}$$

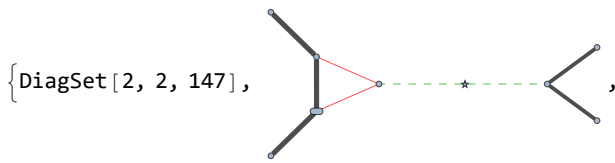

$$\begin{aligned} & \frac{1}{r} \left( \frac{4}{3} \hat{n} \times \vec{S}_1 \cdot \vec{a}_1 (\hat{n} \cdot \vec{v}_2)^2 + \frac{2}{3} \hat{n} \times \vec{S}_1 \cdot \vec{v}_1 (\hat{n} \cdot \vec{v}_2)^2 + \frac{2}{3} \hat{n} \times \vec{S}_1 \cdot \vec{a}_1 (\hat{n} \cdot \vec{v}_2)^2 - \frac{10}{3} \vec{S}_1 \times \vec{a}_1 \cdot \vec{v}_2 \hat{n} \cdot \vec{v}_2 - \frac{5}{3} \vec{S}_1 \times \vec{v}_1 \cdot \vec{v}_2 \hat{n} \cdot \vec{v}_2 - \right. \\ & \quad \frac{5}{3} \vec{S}_1 \times \vec{a}_1 \cdot \vec{v}_2 \hat{n} \cdot \vec{v}_2 + \frac{1}{3} \vec{S}_1 \times \vec{v}_1 \cdot \vec{a}_2 \hat{n} \cdot \vec{a}_1 - \frac{1}{3} \vec{S}_1 \times \vec{v}_1 \cdot \vec{a}_1 \hat{n} \cdot \vec{a}_2 - \frac{2}{3} \hat{n} \times \vec{S}_1 \cdot \vec{v}_1 \hat{n} \cdot \vec{a}_1 \hat{n} \cdot \vec{a}_2 + \frac{5}{3} \vec{S}_1 \times \vec{v}_1 \cdot \vec{a}_2 \hat{n} \cdot \vec{v}_1 + \\ & \quad \frac{5}{3} \vec{S}_1 \times \vec{a}_1 \cdot \vec{a}_2 \hat{n} \cdot \vec{v}_1 - \frac{4}{3} \hat{n} \times \vec{S}_1 \cdot \vec{v}_1 \hat{n} \cdot \vec{a}_2 \hat{n} \cdot \vec{v}_1 - \frac{4}{3} \hat{n} \times \vec{S}_1 \cdot \vec{a}_1 \hat{n} \cdot \vec{a}_2 \hat{n} \cdot \vec{v}_1 + \frac{4}{3} \hat{n} \times \vec{S}_1 \cdot \vec{v}_1 \vec{a}_1 \cdot \vec{a}_2 + \\ & \quad \left. \frac{5}{3} \hat{n} \times \vec{S}_1 \cdot \vec{v}_1 \vec{v}_1 \cdot \vec{a}_2 + \frac{5}{3} \hat{n} \times \vec{S}_1 \cdot \vec{a}_1 \vec{v}_1 \cdot \vec{a}_2 - \frac{2}{3} \hat{n} \times \vec{S}_1 \cdot \vec{a}_1 \vec{v}_2 \cdot \vec{v}_2 - \frac{1}{3} \hat{n} \times \vec{S}_1 \cdot \vec{v}_1 \vec{v}_2 \cdot \vec{v}_2 - \frac{1}{3} \hat{n} \times \vec{S}_1 \cdot \vec{a}_1 \vec{v}_2 \cdot \vec{v}_2 \right) m_1 m_2 G^2 + \\ & \frac{1}{r^2} \left( -\frac{2}{3} \vec{S}_1 \times \vec{v}_1 \cdot \vec{a}_2 (\hat{n} \cdot \vec{v}_1)^2 + \frac{8}{3} \hat{n} \times \vec{S}_1 \cdot \vec{v}_1 \hat{n} \cdot \vec{a}_2 (\hat{n} \cdot \vec{v}_1)^2 - \frac{16}{3} \hat{n} \times \vec{S}_1 \cdot \vec{v}_1 (\hat{n} \cdot \vec{v}_2)^2 \hat{n} \cdot \vec{v}_1 - \right. \\ & \quad \frac{16}{3} \hat{n} \times \vec{S}_1 \cdot \vec{a}_1 (\hat{n} \cdot \vec{v}_2)^2 \hat{n} \cdot \vec{v}_1 + \frac{14}{3} \vec{S}_1 \times \vec{v}_1 \cdot \vec{v}_2 \hat{n} \cdot \vec{v}_2 \hat{n} \cdot \vec{v}_1 + \frac{14}{3} \vec{S}_1 \times \vec{a}_1 \cdot \vec{v}_2 \hat{n} \cdot \vec{v}_2 \hat{n} \cdot \vec{v}_1 - \frac{10}{3} \hat{n} \times \vec{S}_1 \cdot \vec{v}_1 \vec{v}_1 \cdot \vec{a}_2 \hat{n} \cdot \vec{v}_1 + \\ & \quad \frac{4}{3} \hat{n} \times \vec{S}_1 \cdot \vec{v}_1 \vec{v}_2 \cdot \vec{v}_2 \hat{n} \cdot \vec{v}_1 + \frac{4}{3} \hat{n} \times \vec{S}_1 \cdot \vec{a}_1 \vec{v}_2 \cdot \vec{v}_2 \hat{n} \cdot \vec{v}_1 - \frac{2}{3} \vec{S}_1 \times \vec{v}_1 \cdot \vec{a}_1 (\hat{n} \cdot \vec{v}_2)^2 - \frac{8}{3} \hat{n} \times \vec{S}_1 \cdot \vec{v}_1 \hat{n} \cdot \vec{a}_1 (\hat{n} \cdot \vec{v}_2)^2 + \\ & \quad \frac{4}{3} \vec{S}_1 \times \vec{v}_1 \cdot \vec{v}_2 \hat{n} \cdot \vec{a}_1 \hat{n} \cdot \vec{v}_2 - \frac{5}{3} \vec{S}_1 \times \vec{v}_1 \cdot \vec{v}_2 \vec{a}_1 \cdot \vec{v}_2 + \frac{10}{3} \hat{n} \times \vec{S}_1 \cdot \vec{v}_1 \hat{n} \cdot \vec{v}_2 \vec{a}_1 \cdot \vec{v}_2 + \frac{1}{3} \vec{S}_1 \times \vec{v}_1 \cdot \vec{a}_2 \vec{v}_1 \cdot \vec{v}_1 - \\ & \quad \frac{2}{3} \hat{n} \times \vec{S}_1 \cdot \vec{v}_1 \hat{n} \cdot \vec{a}_2 \vec{v}_1 \cdot \vec{v}_1 - \frac{10}{3} \vec{S}_1 \times \vec{v}_1 \cdot \vec{v}_2 \vec{v}_1 \cdot \vec{v}_2 - \frac{10}{3} \vec{S}_1 \times \vec{a}_1 \cdot \vec{v}_2 \vec{v}_1 \cdot \vec{v}_2 + \frac{14}{3} \hat{n} \times \vec{S}_1 \cdot \vec{v}_1 \hat{n} \cdot \vec{v}_2 \vec{v}_1 \cdot \vec{v}_2 + \\ & \quad \left. \frac{14}{3} \hat{n} \times \vec{S}_1 \cdot \vec{a}_1 \hat{n} \cdot \vec{v}_2 \vec{v}_1 \cdot \vec{v}_2 + \frac{1}{3} \vec{S}_1 \times \vec{v}_1 \cdot \vec{a}_1 \vec{v}_2 \cdot \vec{v}_2 + \frac{2}{3} \hat{n} \times \vec{S}_1 \cdot \vec{v}_1 \hat{n} \cdot \vec{a}_1 \vec{v}_2 \cdot \vec{v}_2 \right) m_1 m_2 G^2 + \frac{1}{r^3} \\ & \left( 16 \hat{n} \times \vec{S}_1 \cdot \vec{v}_1 (\hat{n} \cdot \vec{v}_2)^2 (\hat{n} \cdot \vec{v}_1)^2 - \frac{16}{3} \vec{S}_1 \times \vec{v}_1 \cdot \vec{v}_2 \hat{n} \cdot \vec{v}_2 (\hat{n} \cdot \vec{v}_1)^2 - \frac{8}{3} \hat{n} \times \vec{S}_1 \cdot \vec{v}_1 \vec{v}_2 \cdot \vec{v}_2 (\hat{n} \cdot \vec{v}_1)^2 + \right. \\ & \quad \frac{14}{3} \vec{S}_1 \times \vec{v}_1 \cdot \vec{v}_2 \vec{v}_1 \cdot \vec{v}_2 \hat{n} \cdot \vec{v}_1 - \frac{56}{3} \hat{n} \times \vec{S}_1 \cdot \vec{v}_1 \hat{n} \cdot \vec{v}_2 \vec{v}_1 \cdot \vec{v}_2 \hat{n} \cdot \vec{v}_1 + \frac{10}{3} \hat{n} \times \vec{S}_1 \cdot \vec{v}_1 (\vec{v}_1 \cdot \vec{v}_2)^2 - \\ & \quad \left. \frac{8}{3} \hat{n} \times \vec{S}_1 \cdot \vec{v}_1 (\hat{n} \cdot \vec{v}_2)^2 \vec{v}_1 \cdot \vec{v}_1 + \frac{4}{3} \vec{S}_1 \times \vec{v}_1 \cdot \vec{v}_2 \hat{n} \cdot \vec{v}_2 \vec{v}_1 \cdot \vec{v}_1 + \frac{2}{3} \hat{n} \times \vec{S}_1 \cdot \vec{v}_1 \vec{v}_1 \cdot \vec{v}_1 \vec{v}_2 \cdot \vec{v}_2 \right) m_1 m_2 G^2 + \\ & m_1 m_2 \left( \frac{8}{3} \log\left(\frac{r}{R_\theta}\right) \vec{S}_1 \times \vec{a}_1 \cdot \vec{a}_2 - \frac{10}{9} \vec{S}_1 \times \vec{a}_1 \cdot \vec{a}_2 - \frac{5}{9} \vec{S}_1 \times \vec{v}_1 \cdot \vec{a}_2 - \frac{5}{9} \vec{S}_1 \times \vec{a}_1 \cdot \vec{a}_2 + \frac{2}{3} \hat{n} \times \vec{S}_1 \cdot \vec{a}_1 \hat{n} \cdot \vec{a}_2 + \right. \\ & \quad \frac{1}{3} \hat{n} \times \vec{S}_1 \cdot \vec{v}_1 \hat{n} \cdot \vec{a}_2 + \frac{1}{3} \hat{n} \times \vec{S}_1 \cdot \vec{a}_1 \hat{n} \cdot \vec{a}_2 + \frac{4}{3} \vec{S}_1 \times \vec{v}_1 \cdot \vec{a}_2 \log\left(\frac{r}{R_\theta}\right) + \\ & \quad \left. \frac{4}{3} \vec{S}_1 \times \vec{a}_1 \cdot \vec{a}_2 \log\left(\frac{r}{R_\theta}\right) + \frac{-\frac{4}{3} \vec{S}_1 \times \vec{a}_1 \cdot \vec{a}_2 - \frac{2}{3} \vec{S}_1 \times \vec{v}_1 \cdot \vec{a}_2 - \frac{2}{3} \vec{S}_1 \times \vec{a}_1 \cdot \vec{a}_2}{\epsilon_d} \right) G^2 \} \end{aligned}$$

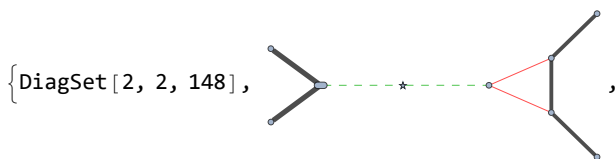

$$\frac{1}{r} G^2 \left( -\frac{1}{3} \hat{n} \times \vec{a}_1 \cdot \vec{S}_1 (\hat{n} \cdot \vec{v}_2)^2 + \frac{1}{3} \hat{n} \times \vec{S}_1 \cdot \vec{v}_1 (\hat{n} \cdot \vec{v}_2)^2 - \frac{2}{3} \hat{n} \times \vec{a}_1 \cdot \vec{S}_1 (\hat{n} \cdot \vec{v}_2)^2 + \frac{5}{6} \vec{a}_1 \times \vec{S}_1 \cdot \vec{v}_2 \hat{n} \cdot \vec{v}_2 - \right.$$

$$\begin{aligned}
& \frac{5}{6} \vec{S}_1 \times \vec{v}_1 \cdot \vec{v}_2 \hat{n} \cdot \vec{v}_2 + \frac{5}{3} \vec{a}_1 \times \vec{S}_1 \cdot \vec{v}_2 \hat{n} \cdot \vec{v}_2 + \frac{7}{24} \vec{a}_2 \times \vec{S}_1 \cdot \vec{v}_1 \hat{n} \cdot \vec{a}_1 - \frac{1}{6} \vec{a}_1 \times \vec{S}_1 \cdot \vec{v}_1 \hat{n} \cdot \vec{a}_2 - \\
& \frac{1}{3} \hat{n} \times \vec{S}_1 \cdot \vec{v}_1 \hat{n} \cdot \vec{a}_1 \hat{n} \cdot \vec{a}_2 + \frac{23}{24} \vec{a}_1 \times \vec{a}_2 \cdot \vec{S}_1 \hat{n} \cdot \vec{v}_1 + \frac{23}{24} \vec{a}_2 \times \vec{S}_1 \cdot \vec{v}_1 \hat{n} \cdot \vec{v}_1 - \frac{2}{3} \hat{n} \times \vec{S}_1 \cdot \vec{v}_1 \hat{n} \cdot \vec{a}_2 \hat{n} \cdot \vec{v}_1 + \\
& \frac{2}{3} \hat{n} \times \vec{a}_1 \cdot \vec{S}_1 \hat{n} \cdot \vec{a}_2 \hat{n} \cdot \vec{v}_1 + \frac{13}{24} \hat{n} \times \vec{S}_1 \cdot \vec{v}_1 \vec{a}_1 \cdot \vec{a}_2 + \frac{17}{24} \hat{n} \times \vec{S}_1 \cdot \vec{v}_1 \vec{a}_2 \cdot \vec{v}_1 - \frac{17}{24} \hat{n} \times \vec{a}_1 \cdot \vec{S}_1 \vec{a}_2 \cdot \vec{v}_1 + \\
& \frac{3}{2} \hat{n} \times \vec{S}_1 \cdot \vec{v}_2 \vec{a}_2 \cdot \vec{v}_2 + \frac{1}{6} \hat{n} \times \vec{a}_1 \cdot \vec{S}_1 \vec{v}_2 \cdot \vec{v}_2 - \frac{1}{6} \hat{n} \times \vec{S}_1 \cdot \vec{v}_1 \vec{v}_2 \cdot \vec{v}_2 + \frac{1}{3} \hat{n} \times \vec{a}_1 \cdot \vec{S}_1 \vec{v}_2 \cdot \vec{v}_2 - \frac{3}{4} \hat{n} \times \vec{a}_2 \cdot \vec{S}_1 \vec{v}_2 \cdot \vec{v}_2 \Big) m_2^2 + \\
& \frac{1}{r^2} G^2 \left( -\frac{7}{12} \vec{a}_2 \times \vec{S}_1 \cdot \vec{v}_1 (\hat{n} \cdot \vec{v}_1)^2 + \frac{4}{3} \hat{n} \times \vec{S}_1 \cdot \vec{v}_1 \hat{n} \cdot \vec{a}_2 (\hat{n} \cdot \vec{v}_1)^2 - \frac{8}{3} \hat{n} \times \vec{S}_1 \cdot \vec{v}_1 (\hat{n} \cdot \vec{v}_2)^2 \hat{n} \cdot \vec{v}_1 + \right. \\
& \frac{8}{3} \hat{n} \times \vec{a}_1 \cdot \vec{S}_1 (\hat{n} \cdot \vec{v}_2)^2 \hat{n} \cdot \vec{v}_1 + \frac{31}{12} \vec{S}_1 \times \vec{v}_1 \cdot \vec{v}_2 \hat{n} \cdot \vec{v}_2 \hat{n} \cdot \vec{v}_1 - \frac{31}{12} \vec{a}_1 \times \vec{S}_1 \cdot \vec{v}_2 \hat{n} \cdot \vec{v}_2 \hat{n} \cdot \vec{v}_1 - \frac{17}{12} \hat{n} \times \vec{S}_1 \cdot \vec{v}_1 \vec{a}_2 \cdot \vec{v}_1 \hat{n} \cdot \vec{v}_1 - \\
& 3 \hat{n} \times \vec{S}_1 \cdot \vec{v}_2 \vec{a}_2 \cdot \vec{v}_2 \hat{n} \cdot \vec{v}_1 + \frac{2}{3} \hat{n} \times \vec{S}_1 \cdot \vec{v}_1 \vec{v}_2 \cdot \vec{v}_2 \hat{n} \cdot \vec{v}_1 - \frac{2}{3} \hat{n} \times \vec{a}_1 \cdot \vec{S}_1 \vec{v}_2 \cdot \vec{v}_2 \hat{n} \cdot \vec{v}_1 + \frac{3}{2} \hat{n} \times \vec{a}_2 \cdot \vec{S}_1 \vec{v}_2 \cdot \vec{v}_2 \hat{n} \cdot \vec{v}_1 - \\
& \frac{1}{3} \vec{a}_1 \times \vec{S}_1 \cdot \vec{v}_1 (\hat{n} \cdot \vec{v}_2)^2 - \frac{4}{3} \hat{n} \times \vec{S}_1 \cdot \vec{v}_1 \hat{n} \cdot \vec{a}_1 (\hat{n} \cdot \vec{v}_2)^2 + \frac{11}{12} \vec{S}_1 \times \vec{v}_1 \cdot \vec{v}_2 \hat{n} \cdot \vec{a}_1 \hat{n} \cdot \vec{v}_2 - \frac{5}{6} \vec{S}_1 \times \vec{v}_1 \cdot \vec{v}_2 \vec{a}_1 \cdot \vec{v}_2 + \\
& \frac{17}{12} \hat{n} \times \vec{S}_1 \cdot \vec{v}_1 \hat{n} \cdot \vec{v}_2 \vec{a}_1 \cdot \vec{v}_2 - \frac{3}{2} \vec{S}_1 \times \vec{v}_1 \cdot \vec{v}_2 \vec{a}_2 \cdot \vec{v}_2 + \frac{7}{24} \vec{a}_2 \times \vec{S}_1 \cdot \vec{v}_1 \vec{v}_1 \cdot \vec{v}_1 - \frac{1}{3} \hat{n} \times \vec{S}_1 \cdot \vec{v}_1 \hat{n} \cdot \vec{a}_2 \vec{v}_1 \cdot \vec{v}_1 - \\
& \frac{5}{3} \vec{S}_1 \times \vec{v}_1 \cdot \vec{v}_2 \vec{v}_1 \cdot \vec{v}_2 + \frac{5}{3} \vec{a}_1 \times \vec{S}_1 \cdot \vec{v}_2 \vec{v}_1 \cdot \vec{v}_2 + \frac{25}{12} \hat{n} \times \vec{S}_1 \cdot \vec{v}_1 \hat{n} \cdot \vec{v}_2 \vec{v}_1 \cdot \vec{v}_2 - \frac{25}{12} \hat{n} \times \vec{a}_1 \cdot \vec{S}_1 \hat{n} \cdot \vec{v}_2 \vec{v}_1 \cdot \vec{v}_2 + \\
& \left. \frac{1}{6} \vec{a}_1 \times \vec{S}_1 \cdot \vec{v}_1 \vec{v}_2 \cdot \vec{v}_2 - \frac{3}{4} \vec{a}_2 \times \vec{S}_1 \cdot \vec{v}_1 \vec{v}_2 \cdot \vec{v}_2 + \frac{1}{3} \hat{n} \times \vec{S}_1 \cdot \vec{v}_1 \hat{n} \cdot \vec{a}_1 \vec{v}_2 \cdot \vec{v}_2 + \frac{3}{2} \hat{n} \times \vec{S}_1 \cdot \vec{v}_2 \hat{n} \cdot \vec{v}_2 \vec{v}_2 \cdot \vec{v}_2 \right) m_2^2 + \\
& \frac{1}{r^3} G^2 \left( 8 \hat{n} \times \vec{S}_1 \cdot \vec{v}_1 (\hat{n} \cdot \vec{v}_2)^2 (\hat{n} \cdot \vec{v}_1)^2 - \frac{11}{3} \vec{S}_1 \times \vec{v}_1 \cdot \vec{v}_2 \hat{n} \cdot \vec{v}_2 (\hat{n} \cdot \vec{v}_1)^2 - \frac{4}{3} \hat{n} \times \vec{S}_1 \cdot \vec{v}_1 \vec{v}_2 \cdot \vec{v}_2 (\hat{n} \cdot \vec{v}_1)^2 + \right. \\
& \frac{31}{12} \vec{S}_1 \times \vec{v}_1 \cdot \vec{v}_2 \vec{v}_1 \cdot \vec{v}_2 \hat{n} \cdot \vec{v}_1 - \frac{25}{3} \hat{n} \times \vec{S}_1 \cdot \vec{v}_1 \hat{n} \cdot \vec{v}_2 \vec{v}_1 \cdot \vec{v}_2 \hat{n} \cdot \vec{v}_1 - 6 \hat{n} \times \vec{S}_1 \cdot \vec{v}_2 \hat{n} \cdot \vec{v}_2 \vec{v}_2 \cdot \vec{v}_2 \hat{n} \cdot \vec{v}_1 + \\
& \frac{17}{12} \hat{n} \times \vec{S}_1 \cdot \vec{v}_1 (\vec{v}_1 \cdot \vec{v}_2)^2 - \frac{4}{3} \hat{n} \times \vec{S}_1 \cdot \vec{v}_1 (\hat{n} \cdot \vec{v}_2)^2 \vec{v}_1 \cdot \vec{v}_1 + \frac{11}{12} \vec{S}_1 \times \vec{v}_1 \cdot \vec{v}_2 \hat{n} \cdot \vec{v}_2 \vec{v}_1 \cdot \vec{v}_1 - \\
& \left. \frac{3}{2} \vec{S}_1 \times \vec{v}_1 \cdot \vec{v}_2 \hat{n} \cdot \vec{v}_2 \vec{v}_2 \cdot \vec{v}_2 + \frac{1}{3} \hat{n} \times \vec{S}_1 \cdot \vec{v}_1 \vec{v}_1 \cdot \vec{v}_1 \vec{v}_2 \cdot \vec{v}_2 + \frac{3}{2} \hat{n} \times \vec{S}_1 \cdot \vec{v}_2 \vec{v}_1 \cdot \vec{v}_2 \vec{v}_2 \cdot \vec{v}_2 \right) m_2^2 + \\
& G^2 \left( \frac{2}{3} \log \left( \frac{r}{R_\theta} \right) \frac{1}{\vec{a}_1 \times \vec{a}_2 \cdot \vec{S}_1} - \frac{4}{9} \frac{1}{\vec{a}_1 \times \vec{a}_2 \cdot \vec{S}_1} - \frac{8}{9} \vec{a}_1 \times \vec{a}_2 \cdot \vec{S}_1 - \frac{4}{9} \vec{a}_2 \times \vec{S}_1 \cdot \vec{v}_1 - \frac{1}{6} \hat{n} \times \vec{a}_1 \cdot \vec{S}_1 \hat{n} \cdot \vec{a}_2 + \right. \\
& \frac{1}{6} \hat{n} \times \vec{S}_1 \cdot \vec{v}_1 \hat{n} \cdot \vec{a}_2 - \frac{1}{3} \hat{n} \times \vec{a}_1 \cdot \vec{S}_1 \hat{n} \cdot \vec{a}_2 + \frac{4}{3} \vec{a}_1 \times \vec{a}_2 \cdot \vec{S}_1 \log \left( \frac{r}{R_\theta} \right) + \\
& \left. \frac{2}{3} \vec{a}_2 \times \vec{S}_1 \cdot \vec{v}_1 \log \left( \frac{r}{R_\theta} \right) + \frac{-\frac{1}{3} \vec{a}_1 \times \vec{a}_2 \cdot \vec{S}_1 - \frac{2}{3} \vec{a}_1 \times \vec{a}_2 \cdot \vec{S}_1 - \frac{1}{3} \vec{a}_2 \times \vec{S}_1 \cdot \vec{v}_1}{\epsilon_d} \right) m_2^2 \Big\}
\end{aligned}$$

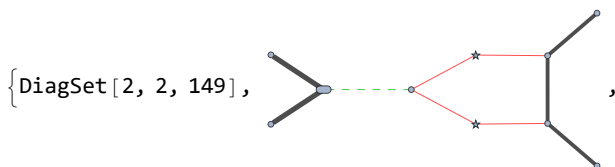

$$\begin{aligned}
& \frac{1}{r} G^2 \left( -\frac{1}{8} \hat{n} \times \vec{S}_1 \cdot \vec{v}_2 (\hat{n} \cdot \vec{a}_2)^2 - \frac{1}{6} \vec{S}_1 \times \vec{v}_1 \cdot \vec{v}_2 \hat{n} \cdot \vec{a}_2 + \frac{1}{12} \vec{a}_1 \times \vec{S}_1 \cdot \vec{v}_2 \hat{n} \cdot \vec{a}_2 + \frac{1}{4} \vec{a}_2 \times \vec{S}_1 \cdot \vec{v}_2 \hat{n} \cdot \vec{a}_2 - \right. \\
& \frac{1}{6} \hat{n} \times \vec{S}_1 \cdot \vec{v}_2 \hat{n} \cdot \vec{a}_1 \hat{n} \cdot \vec{a}_2 - \frac{1}{3} \hat{n} \times \vec{S}_1 \cdot \vec{v}_2 \hat{n} \cdot \vec{v}_1 \hat{n} \cdot \vec{a}_2 + \frac{1}{4} \hat{n} \times \vec{S}_1 \cdot \vec{v}_2 \hat{n} \cdot \vec{v}_2 \hat{n} \cdot \vec{a}_2 - \frac{1}{4} \hat{n} \times \vec{a}_2 \cdot \vec{S}_1 \hat{n} \cdot \vec{v}_2 \hat{n} \cdot \vec{a}_2 + \\
& \left. \frac{1}{8} \hat{n} \times \vec{a}_2 \cdot \vec{S}_1 (\hat{n} \cdot \vec{v}_2)^2 + \frac{1}{24} \hat{n} \times \vec{S}_1 \cdot \vec{v}_2 (\hat{n} \cdot \vec{v}_2)^2 + \frac{1}{8} \hat{n} \times \vec{a}_2 \cdot \vec{S}_1 (\hat{n} \cdot \vec{v}_2)^2 - \frac{1}{12} \vec{S}_1 \times \vec{v}_1 \cdot \vec{v}_2 \hat{n} \cdot \vec{a}_2 + \right.
\end{aligned}$$

[illegible]

$$\left. \frac{1}{6} \vec{a}_2 \times \vec{a}_2 \cdot \vec{S}_1 \log\left(\frac{r}{R_\theta}\right) + \frac{1}{6} \vec{a}_2 \times \vec{S}_1 \cdot \vec{v}_2 \log\left(\frac{r}{R_\theta}\right) + \frac{-\frac{1}{12} \vec{a}_2 \times \vec{S}_1 \cdot \vec{v}_2 - \frac{1}{12} \vec{a}_2 \times \vec{a}_2 \cdot \vec{S}_1 - \frac{1}{12} \vec{a}_2 \times \vec{S}_1 \cdot \vec{v}_2}{\epsilon_d} \right\} m_2^2$$

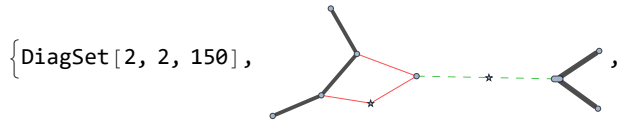

$$\frac{1}{r} G^2 \left( \frac{1}{3} \hat{n} \times \vec{a}_2 \cdot \vec{S}_1 (\hat{n} \cdot \vec{v}_1)^2 - \frac{1}{3} \vec{a}_2 \times \vec{S}_1 \cdot \vec{v}_1 \hat{n} \cdot \vec{v}_1 + \frac{1}{3} \vec{a}_2 \times \vec{S}_1 \cdot \vec{v}_2 \hat{n} \cdot \vec{v}_1 + \frac{1}{3} \vec{a}_2 \times \vec{S}_1 \cdot \vec{v}_2 \hat{n} \cdot \vec{v}_1 - \frac{1}{3} \hat{n} \times \vec{S}_1 \cdot \vec{v}_2 \hat{n} \cdot \vec{a}_2 \hat{n} \cdot \vec{v}_1 - \right.$$

$$\frac{1}{3} \hat{n} \times \vec{a}_2 \cdot \vec{S}_1 \hat{n} \cdot \vec{v}_2 \hat{n} \cdot \vec{v}_1 - \frac{2}{3} \hat{n} \times \vec{a}_2 \cdot \vec{S}_1 \hat{n} \cdot \vec{v}_2 \hat{n} \cdot \vec{v}_1 + \frac{1}{4} \hat{n} \times \vec{a}_2 \cdot \vec{S}_1 (\hat{n} \cdot \vec{v}_2)^2 - \frac{1}{6} \vec{S}_1 \times \vec{v}_1 \cdot \vec{v}_2 \hat{n} \cdot \vec{a}_2 +$$

$$\frac{1}{6} \vec{a}_2 \times \vec{S}_1 \cdot \vec{v}_2 \hat{n} \cdot \vec{a}_1 + \frac{1}{6} \vec{a}_2 \times \vec{S}_1 \cdot \vec{v}_1 \hat{n} \cdot \vec{v}_2 + \frac{1}{6} \vec{a}_1 \times \vec{a}_2 \cdot \vec{S}_1 \hat{n} \cdot \vec{v}_2 + \frac{1}{3} \vec{a}_2 \times \vec{S}_1 \cdot \vec{v}_1 \hat{n} \cdot \vec{v}_2 - \frac{1}{2} \vec{a}_2 \times \vec{S}_1 \cdot \vec{v}_2 \hat{n} \cdot \vec{v}_2 -$$

$$\frac{1}{3} \hat{n} \times \vec{a}_2 \cdot \vec{S}_1 \hat{n} \cdot \vec{a}_1 \hat{n} \cdot \vec{v}_2 + \frac{1}{2} \hat{n} \times \vec{S}_1 \cdot \vec{v}_2 \hat{n} \cdot \vec{a}_2 \hat{n} \cdot \vec{v}_2 + \frac{1}{6} \hat{n} \times \vec{S}_1 \cdot \vec{v}_2 \vec{a}_2 \cdot \vec{v}_1 + \frac{1}{6} \hat{n} \times \vec{a}_2 \cdot \vec{S}_1 \vec{a}_1 \cdot \vec{v}_2 +$$

$$\left. \frac{1}{2} \hat{n} \times \vec{S}_1 \cdot \vec{v}_2 \vec{a}_2 \cdot \vec{v}_2 - \frac{1}{6} \hat{n} \times \vec{a}_2 \cdot \vec{S}_1 \vec{v}_1 \cdot \vec{v}_1 + \frac{1}{6} \hat{n} \times \vec{a}_2 \cdot \vec{S}_1 \vec{v}_1 \cdot \vec{v}_2 + \frac{1}{3} \hat{n} \times \vec{a}_2 \cdot \vec{S}_1 \vec{v}_1 \cdot \vec{v}_2 - \frac{1}{2} \hat{n} \times \vec{a}_2 \cdot \vec{S}_1 \vec{v}_2 \cdot \vec{v}_2 \right) m_2^2 + \frac{1}{r^2}$$

$$G^2 \left( \frac{1}{3} \hat{n} \times \vec{S}_1 \cdot \vec{v}_2 (\hat{n} \cdot \vec{v}_2)^3 + \frac{1}{4} \vec{a}_2 \times \vec{S}_1 \cdot \vec{v}_1 (\hat{n} \cdot \vec{v}_2)^2 - \hat{n} \times \vec{a}_2 \cdot \vec{S}_1 \hat{n} \cdot \vec{v}_1 (\hat{n} \cdot \vec{v}_2)^2 + \frac{4}{3} \hat{n} \times \vec{a}_2 \cdot \vec{S}_1 (\hat{n} \cdot \vec{v}_1)^2 \hat{n} \cdot \vec{v}_2 - \right.$$

$$\frac{1}{2} \vec{S}_1 \times \vec{v}_1 \cdot \vec{v}_2 \hat{n} \cdot \vec{a}_2 \hat{n} \cdot \vec{v}_2 - \frac{2}{3} \vec{a}_2 \times \vec{S}_1 \cdot \vec{v}_1 \hat{n} \cdot \vec{v}_1 \hat{n} \cdot \vec{v}_2 + \vec{a}_2 \times \vec{S}_1 \cdot \vec{v}_2 \hat{n} \cdot \vec{v}_1 \hat{n} \cdot \vec{v}_2 -$$

$$2 \hat{n} \times \vec{S}_1 \cdot \vec{v}_2 \hat{n} \cdot \vec{a}_2 \hat{n} \cdot \vec{v}_1 \hat{n} \cdot \vec{v}_2 + \frac{1}{2} \hat{n} \times \vec{S}_1 \cdot \vec{v}_2 \vec{a}_2 \cdot \vec{v}_1 \hat{n} \cdot \vec{v}_2 - \frac{1}{3} \hat{n} \times \vec{a}_2 \cdot \vec{S}_1 \vec{v}_1 \cdot \vec{v}_1 \hat{n} \cdot \vec{v}_2 +$$

$$\frac{1}{2} \hat{n} \times \vec{a}_2 \cdot \vec{S}_1 \vec{v}_1 \cdot \vec{v}_2 \hat{n} \cdot \vec{v}_2 + \frac{1}{2} \hat{n} \times \vec{S}_1 \cdot \vec{v}_2 \vec{v}_2 \cdot \vec{v}_2 \hat{n} \cdot \vec{v}_2 - \frac{1}{3} \vec{a}_2 \times \vec{S}_1 \cdot \vec{v}_2 (\hat{n} \cdot \vec{v}_1)^2 - \frac{1}{2} \vec{S}_1 \times \vec{v}_1 \cdot \vec{v}_2 \vec{a}_2 \cdot \vec{v}_2 -$$

$$\hat{n} \times \vec{S}_1 \cdot \vec{v}_2 \hat{n} \cdot \vec{v}_1 \vec{a}_2 \cdot \vec{v}_2 + \frac{1}{6} \vec{a}_2 \times \vec{S}_1 \cdot \vec{v}_2 \vec{v}_1 \cdot \vec{v}_1 + \frac{1}{3} \vec{a}_2 \times \vec{S}_1 \cdot \vec{v}_1 \vec{v}_1 \cdot \vec{v}_2 - \frac{1}{2} \vec{a}_2 \times \vec{S}_1 \cdot \vec{v}_2 \vec{v}_1 \cdot \vec{v}_2 +$$

$$\left. \frac{1}{2} \hat{n} \times \vec{S}_1 \cdot \vec{v}_2 \hat{n} \cdot \vec{a}_2 \vec{v}_1 \cdot \vec{v}_2 - \frac{2}{3} \hat{n} \times \vec{a}_2 \cdot \vec{S}_1 \hat{n} \cdot \vec{v}_1 \vec{v}_1 \cdot \vec{v}_2 - \frac{1}{2} \vec{a}_2 \times \vec{S}_1 \cdot \vec{v}_1 \vec{v}_2 \cdot \vec{v}_2 + \hat{n} \times \vec{a}_2 \cdot \vec{S}_1 \hat{n} \cdot \vec{v}_1 \vec{v}_2 \cdot \vec{v}_2 \right) m_2^2 +$$

$$\frac{1}{r^3} G^2 \left( -\frac{1}{3} \vec{S}_1 \times \vec{v}_1 \cdot \vec{v}_2 (\hat{n} \cdot \vec{v}_2)^3 - 2 \hat{n} \times \vec{S}_1 \cdot \vec{v}_2 \hat{n} \cdot \vec{v}_1 (\hat{n} \cdot \vec{v}_2)^3 + \hat{n} \times \vec{S}_1 \cdot \vec{v}_2 \vec{v}_1 \cdot \vec{v}_2 (\hat{n} \cdot \vec{v}_2)^2 - \right.$$

$$\left. \frac{1}{2} \vec{S}_1 \times \vec{v}_1 \cdot \vec{v}_2 \vec{v}_2 \cdot \vec{v}_2 \hat{n} \cdot \vec{v}_2 - 2 \hat{n} \times \vec{S}_1 \cdot \vec{v}_2 \hat{n} \cdot \vec{v}_1 \vec{v}_2 \cdot \vec{v}_2 \hat{n} \cdot \vec{v}_2 + \frac{1}{2} \hat{n} \times \vec{S}_1 \cdot \vec{v}_2 \vec{v}_1 \cdot \vec{v}_2 \vec{v}_2 \cdot \vec{v}_2 \right) m_2^2 +$$

$$G^2 r \left( -\frac{1}{6} \log\left(\frac{r}{R_\theta}\right) \hat{n} \times \vec{a}_2 \cdot \vec{S}_1 + \frac{\hat{n} \times \vec{a}_2 \cdot \vec{S}_1}{12 \epsilon_d} + \frac{11}{72} \hat{n} \times \vec{a}_2 \cdot \vec{S}_1 \right) m_2^2 +$$

$$G^2 \left( -\frac{1}{3} \log\left(\frac{r}{R_\theta}\right) \vec{a}_2 \times \vec{S}_1 \cdot \vec{v}_1 + \frac{11}{36} \vec{a}_2 \times \vec{S}_1 \cdot \vec{v}_1 - \frac{11}{36} \vec{a}_2 \times \vec{S}_1 \cdot \vec{v}_2 + \frac{11}{72} \vec{a}_1 \times \vec{a}_2 \cdot \vec{S}_1 - \frac{11}{72} \vec{a}_2 \times \vec{S}_1 \cdot \vec{v}_2 + \frac{1}{6} \hat{n} \times \vec{S}_1 \cdot \vec{v}_2 \hat{n} \cdot \vec{a}_2 - \right.$$

$$\frac{1}{6} \hat{n} \times \vec{a}_2 \cdot \vec{S}_1 \hat{n} \cdot \vec{a}_1 - \frac{1}{3} \hat{n} \times \vec{a}_2 \cdot \vec{S}_1 \hat{n} \cdot \vec{v}_1 + \frac{1}{6} \hat{n} \times \vec{a}_2 \cdot \vec{S}_1 \hat{n} \cdot \vec{v}_2 + \frac{1}{6} \hat{n} \times \vec{a}_2 \cdot \vec{S}_1 \hat{n} \cdot \vec{v}_2 + \frac{1}{3} \vec{a}_2 \times \vec{S}_1 \cdot \vec{v}_2 \log\left(\frac{r}{R_\theta}\right) -$$

$$\left. \frac{1}{6} \vec{a}_1 \times \vec{a}_2 \cdot \vec{S}_1 \log\left(\frac{r}{R_\theta}\right) + \frac{1}{6} \vec{a}_2 \times \vec{S}_1 \cdot \vec{v}_2 \log\left(\frac{r}{R_\theta}\right) + \frac{\frac{1}{6} \vec{a}_2 \times \vec{S}_1 \cdot \vec{v}_1 - \frac{1}{6} \vec{a}_2 \times \vec{S}_1 \cdot \vec{v}_2 + \frac{1}{12} \vec{a}_1 \times \vec{a}_2 \cdot \vec{S}_1 - \frac{1}{12} \vec{a}_2 \times \vec{S}_1 \cdot \vec{v}_2}{\epsilon_d} \right) m_2^2$$

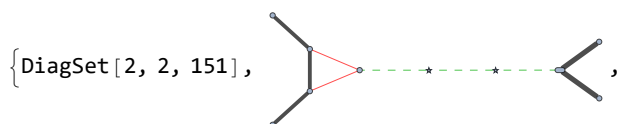

$$\begin{aligned}
& \frac{1}{r} G^2 \left( -\frac{1}{6} \hat{n} \times \vec{a}_2 \cdot \vec{S}_1 (\hat{n} \cdot \vec{v}_1)^2 + \frac{1}{6} \vec{a}_2 \times \vec{S}_1 \cdot \vec{v}_1 \hat{n} \cdot \vec{v}_1 - \frac{1}{6} \vec{a}_2 \times \vec{S}_1 \cdot \vec{v}_2 \hat{n} \cdot \vec{v}_1 - \right. \\
& \quad \frac{1}{3} \hat{n} \times \vec{S}_1 \cdot \vec{v}_2 \hat{n} \cdot \vec{a}_2 \hat{n} \cdot \vec{v}_1 + \frac{2}{3} \hat{n} \times \vec{a}_2 \cdot \vec{S}_1 \hat{n} \cdot \vec{v}_2 \hat{n} \cdot \vec{v}_1 + \frac{1}{6} \hat{n} \times \vec{S}_1 \cdot \vec{v}_2 (\hat{n} \cdot \vec{v}_2)^2 - \frac{1}{12} \vec{a}_2 \times \vec{S}_1 \cdot \vec{v}_2 \hat{n} \cdot \vec{a}_1 - \\
& \quad \frac{1}{6} \vec{S}_1 \times \vec{v}_1 \cdot \vec{v}_2 \hat{n} \cdot \vec{a}_2 + \frac{1}{12} \vec{a}_1 \times \vec{S}_1 \cdot \vec{v}_2 \hat{n} \cdot \vec{a}_2 - \frac{1}{6} \hat{n} \times \vec{S}_1 \cdot \vec{v}_2 \hat{n} \cdot \vec{a}_1 \hat{n} \cdot \vec{a}_2 - \frac{1}{6} \vec{a}_1 \times \vec{a}_2 \cdot \vec{S}_1 \hat{n} \cdot \vec{v}_2 - \\
& \quad \frac{1}{3} \vec{a}_2 \times \vec{S}_1 \cdot \vec{v}_1 \hat{n} \cdot \vec{v}_2 + \frac{1}{3} \hat{n} \times \vec{a}_2 \cdot \vec{S}_1 \hat{n} \cdot \vec{a}_1 \hat{n} \cdot \vec{v}_2 + \frac{1}{12} \hat{n} \times \vec{S}_1 \cdot \vec{v}_2 \vec{a}_1 \cdot \vec{a}_2 - \frac{1}{6} \hat{n} \times \vec{a}_2 \cdot \vec{S}_1 \vec{a}_1 \cdot \vec{v}_2 + \\
& \quad \left. \frac{1}{6} \hat{n} \times \vec{S}_1 \cdot \vec{v}_2 \vec{a}_2 \cdot \vec{v}_1 + \frac{1}{12} \hat{n} \times \vec{a}_2 \cdot \vec{S}_1 \vec{v}_1 \cdot \vec{v}_1 - \frac{1}{3} \hat{n} \times \vec{a}_2 \cdot \vec{S}_1 \vec{v}_1 \cdot \vec{v}_2 - \frac{1}{12} \hat{n} \times \vec{S}_1 \cdot \vec{v}_2 \vec{v}_2 \cdot \vec{v}_2 \right) m_2^2 + \\
& \frac{1}{r^2} G^2 \left( \frac{1}{6} \vec{a}_2 \times \vec{S}_1 \cdot \vec{v}_2 (\hat{n} \cdot \vec{v}_1)^2 + \frac{2}{3} \hat{n} \times \vec{S}_1 \cdot \vec{v}_2 \hat{n} \cdot \vec{a}_2 (\hat{n} \cdot \vec{v}_1)^2 - \frac{4}{3} \hat{n} \times \vec{a}_2 \cdot \vec{S}_1 \hat{n} \cdot \vec{v}_2 (\hat{n} \cdot \vec{v}_1)^2 - \right. \\
& \quad \frac{4}{3} \hat{n} \times \vec{S}_1 \cdot \vec{v}_2 (\hat{n} \cdot \vec{v}_2)^2 \hat{n} \cdot \vec{v}_1 + \frac{1}{3} \vec{S}_1 \times \vec{v}_1 \cdot \vec{v}_2 \hat{n} \cdot \vec{a}_2 \hat{n} \cdot \vec{v}_1 + \frac{2}{3} \vec{a}_2 \times \vec{S}_1 \cdot \vec{v}_1 \hat{n} \cdot \vec{v}_2 \hat{n} \cdot \vec{v}_1 - \\
& \quad \frac{1}{3} \hat{n} \times \vec{S}_1 \cdot \vec{v}_2 \vec{a}_2 \cdot \vec{v}_1 \hat{n} \cdot \vec{v}_1 + \frac{2}{3} \hat{n} \times \vec{a}_2 \cdot \vec{S}_1 \vec{v}_1 \cdot \vec{v}_2 \hat{n} \cdot \vec{v}_1 + \frac{1}{3} \hat{n} \times \vec{S}_1 \cdot \vec{v}_2 \vec{v}_2 \cdot \vec{v}_2 \hat{n} \cdot \vec{v}_1 - \frac{1}{3} \vec{S}_1 \times \vec{v}_1 \cdot \vec{v}_2 (\hat{n} \cdot \vec{v}_2)^2 + \\
& \quad \frac{1}{6} \vec{a}_1 \times \vec{S}_1 \cdot \vec{v}_2 (\hat{n} \cdot \vec{v}_2)^2 - \frac{2}{3} \hat{n} \times \vec{S}_1 \cdot \vec{v}_2 \hat{n} \cdot \vec{a}_1 (\hat{n} \cdot \vec{v}_2)^2 + \frac{1}{3} \hat{n} \times \vec{S}_1 \cdot \vec{v}_2 \hat{n} \cdot \vec{v}_2 \vec{a}_1 \cdot \vec{v}_2 - \frac{1}{6} \vec{S}_1 \times \vec{v}_1 \cdot \vec{v}_2 \vec{a}_2 \cdot \vec{v}_1 - \\
& \quad \frac{1}{12} \vec{a}_2 \times \vec{S}_1 \cdot \vec{v}_2 \vec{v}_1 \cdot \vec{v}_1 - \frac{1}{6} \hat{n} \times \vec{S}_1 \cdot \vec{v}_2 \hat{n} \cdot \vec{a}_2 \vec{v}_1 \cdot \vec{v}_1 + \frac{1}{3} \hat{n} \times \vec{a}_2 \cdot \vec{S}_1 \hat{n} \cdot \vec{v}_2 \vec{v}_1 \cdot \vec{v}_1 - \frac{1}{3} \vec{a}_2 \times \vec{S}_1 \cdot \vec{v}_1 \vec{v}_1 \cdot \vec{v}_2 + \\
& \quad \left. \frac{2}{3} \hat{n} \times \vec{S}_1 \cdot \vec{v}_2 \hat{n} \cdot \vec{v}_2 \vec{v}_1 \cdot \vec{v}_2 + \frac{1}{6} \vec{S}_1 \times \vec{v}_1 \cdot \vec{v}_2 \vec{v}_2 \cdot \vec{v}_2 - \frac{1}{12} \vec{a}_1 \times \vec{S}_1 \cdot \vec{v}_2 \vec{v}_2 \cdot \vec{v}_2 + \frac{1}{6} \hat{n} \times \vec{S}_1 \cdot \vec{v}_2 \hat{n} \cdot \vec{a}_1 \vec{v}_2 \cdot \vec{v}_2 \right) m_2^2 + \\
& \frac{1}{r^3} G^2 \left( 4 \hat{n} \times \vec{S}_1 \cdot \vec{v}_2 (\hat{n} \cdot \vec{v}_2)^2 (\hat{n} \cdot \vec{v}_1)^2 - \frac{2}{3} \hat{n} \times \vec{S}_1 \cdot \vec{v}_2 \vec{v}_2 \cdot \vec{v}_2 (\hat{n} \cdot \vec{v}_1)^2 + \frac{4}{3} \vec{S}_1 \times \vec{v}_1 \cdot \vec{v}_2 (\hat{n} \cdot \vec{v}_2)^2 \hat{n} \cdot \vec{v}_1 - \right. \\
& \quad \frac{8}{3} \hat{n} \times \vec{S}_1 \cdot \vec{v}_2 \hat{n} \cdot \vec{v}_2 \vec{v}_1 \cdot \vec{v}_2 \hat{n} \cdot \vec{v}_1 - \frac{1}{3} \vec{S}_1 \times \vec{v}_1 \cdot \vec{v}_2 \vec{v}_2 \cdot \vec{v}_2 \hat{n} \cdot \vec{v}_1 + \frac{1}{3} \hat{n} \times \vec{S}_1 \cdot \vec{v}_2 (\vec{v}_1 \cdot \vec{v}_2)^2 - \\
& \quad \left. \frac{2}{3} \hat{n} \times \vec{S}_1 \cdot \vec{v}_2 (\hat{n} \cdot \vec{v}_2)^2 \vec{v}_1 \cdot \vec{v}_1 - \frac{2}{3} \vec{S}_1 \times \vec{v}_1 \cdot \vec{v}_2 \hat{n} \cdot \vec{v}_2 \vec{v}_1 \cdot \vec{v}_2 + \frac{1}{6} \hat{n} \times \vec{S}_1 \cdot \vec{v}_2 \vec{v}_1 \cdot \vec{v}_1 \vec{v}_2 \cdot \vec{v}_2 \right) m_2^2 + \\
& G^2 r \left( \frac{1}{12} \log \left( \frac{r}{R_\theta} \right) \hat{n} \times \vec{a}_2 \cdot \vec{S}_1 - \frac{\hat{n} \times \vec{a}_2 \cdot \vec{S}_1}{24 \in_d} - \frac{1}{18} \hat{n} \times \vec{a}_2 \cdot \vec{S}_1 \right) m_2^2 + \\
& G^2 \left( \frac{1}{6} \log \left( \frac{r}{R_\theta} \right) \frac{1}{\vec{a}_2 \times \vec{S}_1 \cdot \vec{v}_1} - \frac{1}{9} \frac{1}{\vec{a}_2 \times \vec{S}_1 \cdot \vec{v}_1} - \frac{1}{18} \frac{1}{\vec{a}_1 \times \vec{a}_2 \cdot \vec{S}_1} + \frac{1}{18} \frac{1}{\vec{a}_2 \times \vec{S}_1 \cdot \vec{v}_2} + \frac{1}{12} \hat{n} \times \vec{a}_2 \cdot \vec{S}_1 \hat{n} \cdot \vec{a}_1 + \right. \\
& \quad \frac{1}{12} \hat{n} \times \vec{S}_1 \cdot \vec{v}_2 \hat{n} \cdot \vec{a}_2 + \frac{1}{6} \hat{n} \times \vec{a}_2 \cdot \vec{S}_1 \hat{n} \cdot \vec{v}_1 - \frac{1}{6} \hat{n} \times \vec{a}_2 \cdot \vec{S}_1 \hat{n} \cdot \vec{v}_2 + \frac{1}{12} \vec{a}_1 \times \vec{a}_2 \cdot \vec{S}_1 \log \left( \frac{r}{R_\theta} \right) - \\
& \quad \left. \frac{1}{12} \vec{a}_2 \times \vec{S}_1 \cdot \vec{v}_2 \log \left( \frac{r}{R_\theta} \right) + \frac{-\frac{1}{12} \frac{1}{\vec{a}_2 \times \vec{S}_1 \cdot \vec{v}_1} - \frac{1}{24} \frac{1}{\vec{a}_1 \times \vec{a}_2 \cdot \vec{S}_1} + \frac{1}{24} \frac{1}{\vec{a}_2 \times \vec{S}_1 \cdot \vec{v}_2}}{\in_d} \right) m_2^2 \Big\}
\end{aligned}$$

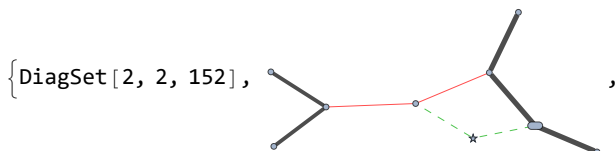

$$\begin{aligned}
& \frac{1}{r} \left( \frac{2}{3} \hat{n} \times \vec{S}_1 \cdot \vec{v}_1 (\hat{n} \cdot \vec{a}_1)^2 + \frac{3}{4} \vec{S}_1 \times \vec{v}_1 \cdot \vec{a}_1 \hat{n} \cdot \vec{a}_1 - \frac{1}{3} \vec{S}_1 \times \vec{v}_1 \cdot \vec{a}_2 \hat{n} \cdot \vec{a}_1 + \frac{2}{3} \hat{n} \times \vec{S}_1 \cdot \vec{v}_1 \hat{n} \cdot \vec{a}_2 \hat{n} \cdot \vec{a}_1 + \frac{4}{3} \hat{n} \times \vec{S}_1 \cdot \vec{v}_1 \hat{n} \cdot \vec{v}_1 \hat{n} \cdot \vec{a}_1 + \right. \\
& \quad \left. \frac{4}{3} \hat{n} \times \vec{S}_1 \cdot \vec{a}_1 \hat{n} \cdot \vec{v}_1 \hat{n} \cdot \vec{a}_1 - 4 \hat{n} \times \vec{S}_1 \cdot \vec{a}_1 (\hat{n} \cdot \vec{v}_1)^2 - 2 \hat{n} \times \vec{S}_1 \cdot \vec{v}_1 (\hat{n} \cdot \vec{v}_1)^2 - 2 \hat{n} \times \vec{S}_1 \cdot \vec{a}_1 (\hat{n} \cdot \vec{v}_1)^2 + \right.
\end{aligned}$$

[illegible]

$\{\text{DiagSet}[2, 2, 153],$

Printed by Wolfram Mathematica Student Edition



$$4 \vec{S_1} \times \vec{v_1} \cdot \vec{v_2} \hat{n} \cdot \vec{v_2} \vec{v_1} \cdot \vec{v_1} - 2 \hat{n} \times \vec{S_1} \cdot \vec{v_1} \vec{v_1} \cdot \vec{v_1} \vec{v_1} \cdot \vec{v_2} + 2 \hat{n} \times \vec{S_1} \cdot \vec{v_1} \vec{v_1} \cdot \vec{v_1} \vec{v_2} \cdot \vec{v_2} \Big) m_1 m_2 G^2 +$$

$$m_1 m_2 \left( \frac{4}{3} \log \left( \frac{r}{R_\theta} \right) \vec{S_1} \times \vec{v_1} \cdot \vec{a_1} - \frac{14}{9} \vec{S_1} \times \vec{v_1} \cdot \vec{a_1} + \frac{14}{9} \vec{S_1} \times \vec{a_1} \cdot \vec{a_1} + \frac{8}{3} \hat{n} \times \vec{S_1} \cdot \vec{a_1} \hat{n} \cdot \vec{a_1} + \frac{4}{3} \hat{n} \times \vec{S_1} \cdot \vec{v_1} \hat{n} \cdot \vec{a_1} + \right.$$

$$\left. \frac{4}{3} \hat{n} \times \vec{S_1} \cdot \vec{a_1} \hat{n} \cdot \vec{a_1} - \frac{4}{3} \vec{S_1} \times \vec{a_1} \cdot \vec{a_1} \log \left( \frac{r}{R_\theta} \right) + \frac{\frac{2}{3} \vec{S_1} \times \vec{a_1} \cdot \vec{a_1} - \frac{2}{3} \vec{S_1} \times \vec{v_1} \cdot \vec{a_1}}{\epsilon_d} \right) G^2 \Big\}$$

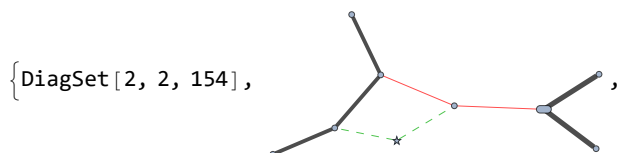

[illegible]

$$\begin{aligned}
& \frac{1}{r^3} G^2 \left( 24 \hat{n} \times \vec{S}_1 \cdot \vec{v}_1 (\hat{n} \cdot \vec{v}_2)^4 - 16 \vec{S}_1 \times \vec{v}_1 \cdot \vec{v}_2 (\hat{n} \cdot \vec{v}_2)^3 - 8 \hat{n} \times \vec{S}_1 \cdot \vec{v}_1 \hat{n} \cdot \vec{v}_1 (\hat{n} \cdot \vec{v}_2)^3 - \right. \\
& 32 \hat{n} \times \vec{S}_1 \cdot \vec{v}_1 (\hat{n} \cdot \vec{v}_1)^2 (\hat{n} \cdot \vec{v}_2)^2 + 4 \vec{S}_1 \times \vec{v}_1 \cdot \vec{v}_2 \hat{n} \cdot \vec{v}_1 (\hat{n} \cdot \vec{v}_2)^2 + \frac{16}{3} \hat{n} \times \vec{S}_1 \cdot \vec{v}_1 \vec{v}_1 \cdot \vec{v}_1 (\hat{n} \cdot \vec{v}_2)^2 + \\
& 4 \hat{n} \times \vec{S}_1 \cdot \vec{v}_1 \vec{v}_1 \cdot \vec{v}_2 (\hat{n} \cdot \vec{v}_2)^2 - 4 \hat{n} \times \vec{S}_1 \cdot \vec{v}_1 \vec{v}_2 \cdot \vec{v}_2 (\hat{n} \cdot \vec{v}_2)^2 + \frac{32}{3} \vec{S}_1 \times \vec{v}_1 \cdot \vec{v}_2 (\hat{n} \cdot \vec{v}_1)^2 \hat{n} \cdot \vec{v}_2 - \\
& \frac{8}{3} \vec{S}_1 \times \vec{v}_1 \cdot \vec{v}_2 \vec{v}_1 \cdot \vec{v}_1 \hat{n} \cdot \vec{v}_2 - 2 \vec{S}_1 \times \vec{v}_1 \cdot \vec{v}_2 \vec{v}_1 \cdot \vec{v}_2 \hat{n} \cdot \vec{v}_2 + \frac{64}{3} \hat{n} \times \vec{S}_1 \cdot \vec{v}_1 \hat{n} \cdot \vec{v}_1 \vec{v}_1 \cdot \vec{v}_2 \hat{n} \cdot \vec{v}_2 + \\
& 2 \vec{S}_1 \times \vec{v}_1 \cdot \vec{v}_2 \vec{v}_2 \cdot \vec{v}_2 \hat{n} \cdot \vec{v}_2 + 8 \hat{n} \times \vec{S}_1 \cdot \vec{v}_1 \hat{n} \cdot \vec{v}_1 \vec{v}_2 \cdot \vec{v}_2 \hat{n} \cdot \vec{v}_2 - \frac{8}{3} \hat{n} \times \vec{S}_1 \cdot \vec{v}_1 (\vec{v}_1 \cdot \vec{v}_2)^2 - \\
& 2 \hat{n} \times \vec{S}_1 \cdot \vec{v}_1 (\vec{v}_2 \cdot \vec{v}_2)^2 - \frac{16}{3} \vec{S}_1 \times \vec{v}_1 \cdot \vec{v}_2 \hat{n} \cdot \vec{v}_1 \vec{v}_1 \cdot \vec{v}_2 - \frac{32}{3} \hat{n} \times \vec{S}_1 \cdot \vec{v}_1 (\hat{n} \cdot \vec{v}_1)^2 \vec{v}_2 \cdot \vec{v}_2 - \\
& \left. 2 \vec{S}_1 \times \vec{v}_1 \cdot \vec{v}_2 \hat{n} \cdot \vec{v}_1 \vec{v}_2 \cdot \vec{v}_2 + \frac{8}{3} \hat{n} \times \vec{S}_1 \cdot \vec{v}_1 \vec{v}_1 \cdot \vec{v}_1 \vec{v}_2 \cdot \vec{v}_2 - 2 \hat{n} \times \vec{S}_1 \cdot \vec{v}_1 \vec{v}_1 \cdot \vec{v}_2 \vec{v}_2 \cdot \vec{v}_2 \right) m_2^2 + \\
& G^2 \left( \frac{4}{3} \log \left( \frac{r}{R_\theta} \right) \frac{1}{\vec{a}_1 \times \vec{a}_2 \cdot \vec{S}_1} - \frac{14}{9} \frac{1}{\vec{a}_1 \times \vec{a}_2 \cdot \vec{S}_1} - \frac{28}{9} \frac{1}{\vec{a}_1 \times \vec{a}_2 \cdot \vec{S}_1} - \frac{14}{9} \frac{2}{\vec{a}_2 \times \vec{S}_1 \cdot \vec{v}_1} - \frac{4}{3} \hat{n} \times \frac{1}{\vec{a}_1} \cdot \vec{S}_1 \hat{n} \cdot \vec{a}_2 + \right. \\
& \frac{4}{3} \hat{n} \times \vec{S}_1 \cdot \vec{v}_1 \hat{n} \cdot \vec{a}_2 - \frac{8}{3} \hat{n} \times \vec{a}_1 \cdot \vec{S}_1 \hat{n} \cdot \vec{a}_2 + \frac{8}{3} \vec{a}_1 \times \vec{a}_2 \cdot \vec{S}_1 \log \left( \frac{r}{R_\theta} \right) + \\
& \left. \frac{4}{3} \vec{a}_2 \times \vec{S}_1 \cdot \vec{v}_1 \log \left( \frac{r}{R_\theta} \right) + \frac{-\frac{2}{3} \frac{1}{\vec{a}_1 \times \vec{a}_2 \cdot \vec{S}_1} - \frac{4}{3} \frac{1}{\vec{a}_1 \times \vec{a}_2 \cdot \vec{S}_1} - \frac{2}{3} \frac{2}{\vec{a}_2 \times \vec{S}_1 \cdot \vec{v}_1}}{\epsilon_d} \right) m_2^2 \}
\end{aligned}$$

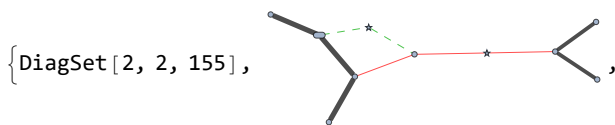

$$\begin{aligned}
& \frac{1}{r} \left( \frac{1}{8} \vec{S}_1 \times \vec{v}_1 \cdot \vec{v}_2 \hat{n} \cdot \frac{1}{\vec{a}_1} - \frac{1}{4} \hat{n} \times \vec{S}_1 \cdot \vec{v}_1 \hat{n} \cdot \vec{v}_2 \hat{n} \cdot \frac{1}{\vec{a}_1} - \frac{1}{8} \frac{1}{\vec{S}_1 \times \vec{v}_1 \cdot \vec{v}_2} \hat{n} \cdot \vec{a}_1 + \frac{1}{12} \vec{S}_1 \times \vec{a}_1 \cdot \vec{v}_2 \hat{n} \cdot \vec{a}_1 + \frac{1}{2} \frac{1}{\vec{S}_1 \times \vec{v}_1 \cdot \vec{v}_2} \hat{n} \cdot \vec{a}_2 + \right. \\
& \frac{1}{2} \vec{S}_1 \times \vec{a}_1 \cdot \vec{v}_2 \hat{n} \cdot \vec{a}_2 - \frac{11}{24} \frac{1}{\vec{S}_1 \times \vec{a}_1 \cdot \vec{v}_2} \hat{n} \cdot \vec{v}_1 - \frac{1}{4} \frac{2}{\vec{S}_1 \times \vec{v}_1 \cdot \vec{v}_2} \hat{n} \cdot \vec{v}_1 - \frac{1}{24} \vec{S}_1 \times \vec{a}_1 \cdot \vec{v}_2 \hat{n} \cdot \vec{v}_1 - \frac{1}{6} \vec{S}_1 \times \vec{v}_1 \cdot \vec{a}_2 \hat{n} \cdot \vec{v}_1 + \\
& \frac{1}{3} \hat{n} \times \vec{S}_1 \cdot \vec{v}_1 \hat{n} \cdot \frac{1}{\vec{a}_2} \hat{n} \cdot \vec{v}_1 + \frac{1}{3} \frac{1}{\vec{S}_1 \times \vec{v}_1 \cdot \vec{a}_1} \hat{n} \cdot \vec{v}_2 + \frac{1}{2} \frac{1}{\vec{S}_1 \times \vec{v}_1 \cdot \vec{a}_2} \hat{n} \cdot \vec{v}_2 + \frac{1}{2} \vec{S}_1 \times \vec{a}_1 \cdot \vec{a}_2 \hat{n} \cdot \vec{v}_2 + \\
& \frac{1}{6} \vec{S}_1 \times \vec{v}_1 \cdot \frac{1}{\vec{a}_1} \hat{n} \cdot \vec{v}_2 + \frac{1}{4} \hat{n} \times \vec{S}_1 \cdot \vec{v}_1 \hat{n} \cdot \vec{a}_1 \hat{n} \cdot \vec{v}_2 - \frac{1}{6} \hat{n} \times \vec{S}_1 \cdot \vec{a}_1 \hat{n} \cdot \vec{a}_1 \hat{n} \cdot \vec{v}_2 - \hat{n} \times \vec{S}_1 \cdot \vec{v}_1 \hat{n} \cdot \vec{a}_2 \hat{n} \cdot \vec{v}_2 - \\
& \hat{n} \times \vec{S}_1 \cdot \vec{a}_1 \hat{n} \cdot \vec{a}_2 \hat{n} \cdot \vec{v}_2 + \frac{11}{12} \hat{n} \times \vec{S}_1 \cdot \vec{a}_1 \hat{n} \cdot \vec{v}_1 \hat{n} \cdot \vec{v}_2 + \frac{1}{2} \hat{n} \times \vec{S}_1 \cdot \vec{v}_1 \hat{n} \cdot \vec{v}_1 \hat{n} \cdot \vec{v}_2 + \frac{1}{12} \hat{n} \times \vec{S}_1 \cdot \vec{a}_1 \hat{n} \cdot \vec{v}_1 \hat{n} \cdot \vec{v}_2 + \\
& \frac{1}{8} \hat{n} \times \vec{S}_1 \cdot \vec{v}_1 \frac{1}{\vec{a}_1} \cdot \vec{v}_2 - \frac{1}{8} \hat{n} \times \vec{S}_1 \cdot \vec{v}_1 \vec{a}_1 \cdot \vec{v}_2 + \frac{1}{12} \hat{n} \times \vec{S}_1 \cdot \vec{a}_1 \vec{a}_1 \cdot \vec{v}_2 - \frac{1}{6} \hat{n} \times \vec{S}_1 \cdot \vec{v}_1 \vec{v}_1 \cdot \frac{1}{\vec{a}_2} - \frac{11}{24} \hat{n} \times \vec{S}_1 \cdot \vec{a}_1 \vec{v}_1 \cdot \vec{v}_2 - \\
& \frac{1}{4} \hat{n} \times \vec{S}_1 \cdot \frac{2}{\vec{v}_1 \vec{v}_1 \cdot \vec{v}_2} - \frac{1}{24} \hat{n} \times \vec{S}_1 \cdot \frac{1}{\vec{a}_1} \vec{v}_1 \cdot \vec{v}_2 + \frac{1}{2} \hat{n} \times \vec{S}_1 \cdot \vec{v}_1 \vec{v}_2 \cdot \vec{a}_2 + \frac{1}{2} \hat{n} \times \vec{S}_1 \cdot \vec{a}_1 \vec{v}_2 \cdot \vec{a}_2 \Big) m_1 m_2 G^2 + \\
& \frac{1}{r^2} \left( -\frac{4}{3} \hat{n} \times \vec{S}_1 \cdot \vec{v}_1 (\hat{n} \cdot \vec{v}_2)^3 - \frac{4}{3} \hat{n} \times \vec{S}_1 \cdot \vec{a}_1 (\hat{n} \cdot \vec{v}_2)^3 + \vec{S}_1 \times \vec{v}_1 \cdot \vec{v}_2 (\hat{n} \cdot \vec{v}_2)^2 + \vec{S}_1 \times \vec{a}_1 \cdot \vec{v}_2 (\hat{n} \cdot \vec{v}_2)^2 - \right. \\
& \frac{3}{2} \hat{n} \times \vec{S}_1 \cdot \vec{v}_1 (\hat{n} \cdot \vec{v}_1)^2 \hat{n} \cdot \vec{v}_2 + \frac{1}{6} \hat{n} \times \vec{S}_1 \cdot \vec{a}_1 (\hat{n} \cdot \vec{v}_1)^2 \hat{n} \cdot \vec{v}_2 - \frac{5}{12} \vec{S}_1 \times \vec{v}_1 \cdot \vec{a}_1 \hat{n} \cdot \vec{v}_1 \hat{n} \cdot \vec{v}_2 - \\
& \vec{S}_1 \times \vec{v}_1 \cdot \vec{a}_2 \hat{n} \cdot \vec{v}_1 \hat{n} \cdot \vec{v}_2 + 2 \hat{n} \times \vec{S}_1 \cdot \vec{v}_1 \hat{n} \cdot \vec{a}_1 \hat{n} \cdot \vec{v}_1 \hat{n} \cdot \vec{v}_2 + 4 \hat{n} \times \vec{S}_1 \cdot \vec{v}_1 \hat{n} \cdot \vec{a}_2 \hat{n} \cdot \vec{v}_1 \hat{n} \cdot \vec{v}_2 + \\
& \frac{1}{4} \hat{n} \times \vec{S}_1 \cdot \vec{v}_1 \vec{v}_1 \cdot \vec{a}_1 \hat{n} \cdot \vec{v}_2 - \hat{n} \times \vec{S}_1 \cdot \vec{v}_1 \vec{v}_1 \cdot \vec{a}_2 \hat{n} \cdot \vec{v}_2 + \frac{3}{4} \hat{n} \times \vec{S}_1 \cdot \vec{v}_1 \vec{v}_1 \cdot \vec{v}_1 \hat{n} \cdot \vec{v}_2 + \frac{1}{3} \hat{n} \times \vec{S}_1 \cdot \vec{a}_1 \vec{v}_1 \cdot \vec{v}_1 \hat{n} \cdot \vec{v}_2 + \\
& \left. \hat{n} \times \vec{S}_1 \cdot \vec{v}_1 \vec{v}_2 \cdot \vec{v}_2 \hat{n} \cdot \vec{v}_2 + \hat{n} \times \vec{S}_1 \cdot \vec{a}_1 \vec{v}_2 \cdot \vec{v}_2 \hat{n} \cdot \vec{v}_2 + \frac{3}{8} \frac{1}{\vec{S}_1 \times \vec{v}_1 \cdot \vec{v}_2} (\hat{n} \cdot \vec{v}_1)^2 - \frac{1}{24} \vec{S}_1 \times \vec{a}_1 \cdot \vec{v}_2 (\hat{n} \cdot \vec{v}_1)^2 - \right)
\end{aligned}$$

$$\begin{aligned} & \frac{1}{2} \vec{S}_1 \times \vec{v}_1 \cdot \vec{v}_2 \hat{n} \cdot \vec{a}_1 \hat{n} \cdot \vec{v}_1 - \vec{S}_1 \times \vec{v}_1 \cdot \vec{v}_2 \hat{n} \cdot \vec{a}_2 \hat{n} \cdot \vec{v}_1 - \frac{1}{2} \hat{n} \times \vec{S}_1 \cdot \vec{v}_1 \hat{n} \cdot \vec{v}_1 \vec{a}_1 \cdot \vec{v}_2 - \frac{1}{8} \vec{S}_1 \times \vec{v}_1 \cdot \vec{v}_2 \vec{v}_1 \cdot \vec{a}_1 + \\ & \frac{1}{2} \vec{S}_1 \times \vec{v}_1 \cdot \vec{v}_2 \vec{v}_1 \cdot \vec{a}_2 - \frac{3}{8} \frac{\vec{S}_1}{\vec{S}_1 \times \vec{v}_1 \cdot \vec{v}_2 \vec{v}_1 \cdot \vec{v}_1} - \frac{1}{6} \vec{S}_1 \times \vec{a}_1 \cdot \vec{v}_2 \vec{v}_1 \cdot \vec{v}_1 + \frac{5}{24} \vec{S}_1 \times \vec{v}_1 \cdot \vec{a}_1 \vec{v}_1 \cdot \vec{v}_2 + \\ & \frac{1}{2} \vec{S}_1 \times \vec{v}_1 \cdot \vec{a}_2 \vec{v}_1 \cdot \vec{v}_2 - \frac{1}{2} \hat{n} \times \vec{S}_1 \cdot \vec{v}_1 \hat{n} \cdot \vec{a}_1 \vec{v}_1 \cdot \vec{v}_2 - \hat{n} \times \vec{S}_1 \cdot \vec{v}_1 \hat{n} \cdot \vec{a}_2 \vec{v}_1 \cdot \vec{v}_2 + \frac{3}{4} \hat{n} \times \vec{S}_1 \cdot \vec{v}_1 \hat{n} \cdot \vec{v}_1 \vec{v}_1 \cdot \vec{v}_2 - \\ & \frac{1}{12} \hat{n} \times \vec{S}_1 \cdot \vec{a}_1 \hat{n} \cdot \vec{v}_1 \vec{v}_1 \cdot \vec{v}_2 - \hat{n} \times \vec{S}_1 \cdot \vec{v}_1 \hat{n} \cdot \vec{v}_1 \vec{v}_2 \cdot \vec{a}_2 - \frac{1}{2} \frac{\vec{S}_1}{\vec{S}_1 \times \vec{v}_1 \cdot \vec{v}_2 \vec{v}_2 \cdot \vec{v}_2} - \frac{1}{2} \vec{S}_1 \times \vec{a}_1 \cdot \vec{v}_2 \vec{v}_2 \cdot \vec{v}_2 \left) m_1 m_2 G^2 + \frac{1}{r^3} \right. \\ & \left( \frac{1}{2} \vec{S}_1 \times \vec{v}_1 \cdot \vec{v}_2 (\hat{n} \cdot \vec{v}_1)^3 - 3 \hat{n} \times \vec{S}_1 \cdot \vec{v}_1 \hat{n} \cdot \vec{v}_2 (\hat{n} \cdot \vec{v}_1)^3 + \frac{3}{2} \hat{n} \times \vec{S}_1 \cdot \vec{v}_1 \vec{v}_1 \cdot \vec{v}_2 (\hat{n} \cdot \vec{v}_1)^2 + 8 \hat{n} \times \vec{S}_1 \cdot \vec{v}_1 (\hat{n} \cdot \vec{v}_2)^3 \hat{n} \cdot \vec{v}_1 - \right. \\ & 4 \vec{S}_1 \times \vec{v}_1 \cdot \vec{v}_2 (\hat{n} \cdot \vec{v}_2)^2 \hat{n} \cdot \vec{v}_1 + \vec{S}_1 \times \vec{v}_1 \cdot \vec{v}_2 \vec{v}_2 \cdot \vec{v}_2 \hat{n} \cdot \vec{v}_1 - 4 \hat{n} \times \vec{S}_1 \cdot \vec{v}_1 \hat{n} \cdot \vec{v}_2 \vec{v}_2 \cdot \vec{v}_2 \hat{n} \cdot \vec{v}_1 - \\ & \left. 4 \hat{n} \times \vec{S}_1 \cdot \vec{v}_1 (\hat{n} \cdot \vec{v}_2)^2 \vec{v}_1 \cdot \vec{v}_2 + 2 \vec{S}_1 \times \vec{v}_1 \cdot \vec{v}_2 \hat{n} \cdot \vec{v}_2 \vec{v}_1 \cdot \vec{v}_2 + \hat{n} \times \vec{S}_1 \cdot \vec{v}_1 \vec{v}_1 \cdot \vec{v}_2 \vec{v}_2 \cdot \vec{v}_2 \right) m_1 m_2 G^2 + \\ & m_1 m_2 \left( -\frac{1}{6} \log \left( \frac{r}{R_\theta} \right) \frac{\vec{S}_1}{\vec{S}_1 \times \vec{a}_1 \cdot \vec{v}_2} + \frac{11}{72} \frac{\vec{S}_1}{\vec{S}_1 \times \vec{a}_1 \cdot \vec{v}_2} + \frac{11}{72} \frac{\vec{S}_1}{\vec{S}_1 \times \vec{v}_1 \cdot \vec{a}_2} + \frac{11}{72} \frac{\vec{S}_1^2}{\vec{S}_1 \times \vec{a}_1 \cdot \vec{v}_2} + \frac{11}{72} \vec{S}_1 \times \vec{a}_1 \cdot \frac{1}{\vec{a}_2} - \frac{1}{6} \hat{n} \times \vec{S}_1 \cdot \vec{v}_1 \hat{n} \cdot \frac{1}{\vec{a}_2} - \right. \\ & \frac{1}{6} \hat{n} \times \vec{S}_1 \cdot \vec{a}_1 \hat{n} \cdot \frac{1}{\vec{a}_2} - \frac{1}{6} \hat{n} \times \vec{S}_1 \cdot \vec{a}_1 \hat{n} \cdot \vec{v}_2 - \frac{1}{6} \hat{n} \times \vec{S}_1 \cdot \vec{a}_1 \hat{n} \cdot \vec{v}_2 - \frac{1}{6} \frac{\vec{S}_1}{\vec{S}_1 \times \vec{v}_1 \cdot \vec{a}_2} \log \left( \frac{r}{R_\theta} \right) - \frac{1}{6} \frac{\vec{S}_1^2}{\vec{S}_1 \times \vec{a}_1 \cdot \vec{v}_2} \log \left( \frac{r}{R_\theta} \right) - \\ & \left. \frac{1}{6} \vec{S}_1 \times \vec{a}_1 \cdot \frac{1}{\vec{a}_2} \log \left( \frac{r}{R_\theta} \right) + \frac{\frac{1}{12} \vec{S}_1 \times \vec{a}_1 \cdot \vec{v}_2 + \frac{1}{12} \vec{S}_1 \times \vec{v}_1 \cdot \vec{a}_2 + \frac{1}{12} \vec{S}_1 \times \vec{a}_1 \cdot \vec{v}_2 + \frac{1}{12} \vec{S}_1 \times \vec{a}_1 \cdot \frac{1}{\vec{a}_2}}{e_d} \right) G^2 \Big\} \end{aligned}$$

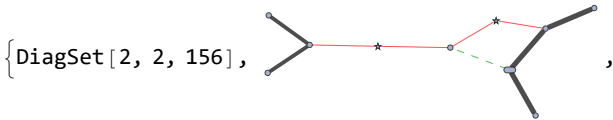

$$\begin{aligned} & \frac{1}{r} \left( \frac{2}{3} \hat{n} \times \vec{S}_1 \cdot \vec{v}_1 (\hat{n} \cdot \vec{v}_2)^2 - \frac{1}{3} \hat{n} \times \vec{S}_1 \cdot \vec{a}_1 (\hat{n} \cdot \vec{v}_2)^2 + \frac{1}{3} \vec{S}_1 \times \vec{v}_1 \cdot \vec{a}_1 \hat{n} \cdot \vec{v}_2 - \frac{1}{2} \vec{S}_1 \times \vec{v}_1 \cdot \vec{a}_2 \hat{n} \cdot \vec{v}_2 - \frac{1}{3} \vec{S}_1 \times \vec{v}_1 \cdot \vec{v}_2 \hat{n} \cdot \vec{v}_2 + \right. \\ & \quad \frac{1}{3} \vec{S}_1 \times \vec{a}_1 \cdot \vec{v}_2 \hat{n} \cdot \vec{v}_2 - \frac{1}{2} \vec{S}_1 \times \vec{a}_1 \cdot \vec{a}_2 \hat{n} \cdot \vec{v}_2 + \frac{1}{6} \vec{S}_1 \times \vec{v}_1 \cdot \vec{a}_1 \hat{n} \cdot \vec{v}_2 - \frac{1}{12} \hat{n} \times \vec{S}_1 \cdot \vec{v}_1 \hat{n} \cdot \vec{a}_1 \hat{n} \cdot \vec{v}_2 + \\ & \quad \frac{1}{12} \hat{n} \times \vec{S}_1 \cdot \vec{v}_1 \hat{n} \cdot \vec{a}_1 \hat{n} \cdot \vec{v}_2 + \frac{1}{6} \hat{n} \times \vec{S}_1 \cdot \vec{a}_1 \hat{n} \cdot \vec{a}_1 \hat{n} \cdot \vec{v}_2 + \hat{n} \times \vec{S}_1 \cdot \vec{v}_1 \hat{n} \cdot \vec{a}_2 \hat{n} \cdot \vec{v}_2 + \hat{n} \times \vec{S}_1 \cdot \vec{a}_1 \hat{n} \cdot \vec{a}_2 \hat{n} \cdot \vec{v}_2 + \\ & \quad \frac{3}{4} \hat{n} \times \vec{S}_1 \cdot \vec{a}_1 \hat{n} \cdot \vec{v}_1 \hat{n} \cdot \vec{v}_2 + \frac{1}{6} \hat{n} \times \vec{S}_1 \cdot \vec{v}_1 \hat{n} \cdot \vec{v}_1 \hat{n} \cdot \vec{v}_2 + \frac{1}{4} \hat{n} \times \vec{S}_1 \cdot \vec{a}_1 \hat{n} \cdot \vec{v}_1 \hat{n} \cdot \vec{v}_2 + \frac{1}{24} \vec{S}_1 \times \vec{v}_1 \cdot \vec{v}_2 \hat{n} \cdot \vec{a}_1 - \\ & \quad \frac{1}{24} \vec{S}_1 \times \vec{v}_1 \cdot \vec{v}_2 \hat{n} \cdot \vec{a}_1 - \frac{1}{12} \vec{S}_1 \times \vec{a}_1 \cdot \vec{v}_2 \hat{n} \cdot \vec{a}_1 - \frac{1}{2} \vec{S}_1 \times \vec{v}_1 \cdot \vec{v}_2 \hat{n} \cdot \vec{a}_2 - \frac{1}{2} \vec{S}_1 \times \vec{a}_1 \cdot \vec{v}_2 \hat{n} \cdot \vec{a}_2 + \frac{1}{6} \vec{S}_1 \times \vec{v}_1 \cdot \vec{a}_1 \hat{n} \cdot \vec{a}_2 - \\ & \quad \frac{3}{8} \vec{S}_1 \times \vec{a}_1 \cdot \vec{v}_2 \hat{n} \cdot \vec{v}_1 + \frac{1}{6} \vec{S}_1 \times \vec{v}_1 \cdot \vec{a}_2 \hat{n} \cdot \vec{v}_1 - \frac{1}{12} \vec{S}_1 \times \vec{v}_1 \cdot \vec{v}_2 \hat{n} \cdot \vec{v}_1 - \frac{1}{8} \vec{S}_1 \times \vec{a}_1 \cdot \vec{v}_2 \hat{n} \cdot \vec{v}_1 - \frac{1}{6} \vec{S}_1 \times \vec{a}_1 \cdot \vec{a}_2 \hat{n} \cdot \vec{v}_1 + \\ & \quad \frac{1}{6} \vec{S}_1 \times \vec{v}_1 \cdot \vec{a}_2 \hat{n} \cdot \vec{v}_1 - \frac{1}{3} \hat{n} \times \vec{S}_1 \cdot \vec{v}_1 \hat{n} \cdot \vec{a}_2 \hat{n} \cdot \vec{v}_1 - \frac{1}{3} \hat{n} \times \vec{S}_1 \cdot \vec{v}_1 \hat{n} \cdot \vec{a}_2 \hat{n} \cdot \vec{v}_1 + \frac{1}{3} \hat{n} \times \vec{S}_1 \cdot \vec{a}_1 \hat{n} \cdot \vec{a}_2 \hat{n} \cdot \vec{v}_1 + \\ & \quad \frac{1}{24} \hat{n} \times \vec{S}_1 \cdot \vec{v}_1 \vec{a}_1 \cdot \vec{v}_2 - \frac{1}{24} \hat{n} \times \vec{S}_1 \cdot \vec{v}_1 \vec{a}_1 \cdot \vec{v}_2 - \frac{1}{12} \hat{n} \times \vec{S}_1 \cdot \vec{a}_1 \vec{a}_1 \cdot \vec{v}_2 + \frac{1}{6} \hat{n} \times \vec{S}_1 \cdot \vec{v}_1 \vec{v}_1 \cdot \vec{a}_2 + \\ & \quad \frac{1}{6} \hat{n} \times \vec{S}_1 \cdot \vec{v}_1 \vec{v}_1 \cdot \vec{a}_2 - \frac{1}{6} \hat{n} \times \vec{S}_1 \cdot \vec{a}_1 \vec{v}_1 \cdot \vec{a}_2 - \frac{3}{8} \hat{n} \times \vec{S}_1 \cdot \vec{a}_1 \vec{v}_1 \cdot \vec{v}_2 - \frac{1}{12} \hat{n} \times \vec{S}_1 \cdot \vec{v}_1 \vec{v}_1 \cdot \vec{v}_2 - \frac{1}{8} \hat{n} \times \vec{S}_1 \cdot \vec{a}_1 \vec{v}_1 \cdot \vec{v}_2 - \\ & \quad \left. \frac{1}{2} \hat{n} \times \vec{S}_1 \cdot \vec{v}_1 \vec{v}_2 \cdot \vec{a}_2 - \frac{1}{2} \hat{n} \times \vec{S}_1 \cdot \vec{a}_1 \vec{v}_2 \cdot \vec{a}_2 - \frac{1}{6} \hat{n} \times \vec{S}_1 \cdot \vec{v}_1 \vec{v}_2 \cdot \vec{v}_2 + \frac{1}{6} \hat{n} \times \vec{S}_1 \cdot \vec{a}_1 \vec{v}_2 \cdot \vec{v}_2 \right) m_1 m_2 G^2 + \\ & \frac{1}{r^2} \left( \frac{4}{3} \hat{n} \times \vec{S}_1 \cdot \vec{v}_1 (\hat{n} \cdot \vec{v}_2)^3 + \frac{4}{3} \hat{n} \times \vec{S}_1 \cdot \vec{a}_1 (\hat{n} \cdot \vec{v}_2)^3 - \vec{S}_1 \times \vec{v}_1 \cdot \vec{v}_2 (\hat{n} \cdot \vec{v}_2)^2 - \vec{S}_1 \times \vec{a}_1 \cdot \vec{v}_2 (\hat{n} \cdot \vec{v}_2)^2 + \right. \\ & \quad \left. \frac{1}{3} \vec{S}_1 \times \vec{v}_1 \cdot \vec{a}_1 (\hat{n} \cdot \vec{v}_2)^2 - \frac{4}{3} \hat{n} \times \vec{S}_1 \cdot \vec{v}_1 \hat{n} \cdot \vec{v}_1 (\hat{n} \cdot \vec{v}_2)^2 + \frac{4}{3} \hat{n} \times \vec{S}_1 \cdot \vec{a}_1 \hat{n} \cdot \vec{v}_1 (\hat{n} \cdot \vec{v}_2)^2 - \frac{5}{6} \hat{n} \times \vec{S}_1 \cdot \vec{v}_1 (\hat{n} \cdot \vec{v}_1)^2 \hat{n} \cdot \vec{v}_2 - \right. \end{aligned}$$

DiagSet[2, 2, 157],

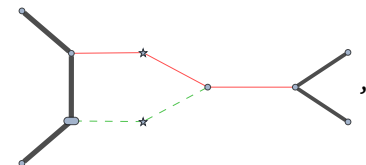

Printed by Wolfram Mathematica Student Edition

[illegible]

$\epsilon_a$

$$\frac{1}{r^2}$$

$$\begin{aligned}
& \frac{2}{3} \hat{n} \times \vec{S}_1 \cdot \vec{a}_1 (\hat{n} \cdot \vec{v}_2)^3 - \frac{1}{\vec{S}_1 \times \vec{v}_1 \cdot \vec{v}_2} (\hat{n} \cdot \vec{v}_2)^2 - \frac{1}{2} \vec{S}_1 \times \vec{a}_1 \cdot \vec{v}_2 (\hat{n} \cdot \vec{v}_2)^2 - \frac{1}{6} \vec{S}_1 \times \vec{v}_1 \cdot \vec{a}_1 (\hat{n} \cdot \vec{v}_2)^2 - \\
& \frac{1}{3} \hat{n} \times \vec{S}_1 \cdot \vec{v}_1 \hat{n} \cdot \vec{a}_1 (\hat{n} \cdot \vec{v}_2)^2 + \frac{1}{6} \vec{S}_1 \times \vec{v}_1 \cdot \vec{v}_2 \hat{n} \cdot \vec{a}_1 \hat{n} \cdot \vec{v}_2 - \frac{1}{12} \vec{S}_1 \times \vec{v}_1 \cdot \vec{v}_2 \vec{a}_1 \cdot \vec{v}_2 + \frac{1}{6} \hat{n} \times \vec{S}_1 \cdot \vec{v}_1 \hat{n} \cdot \vec{v}_2 \vec{a}_1 \cdot \vec{v}_2 + \\
& \frac{1}{4} \vec{S}_1 \times \vec{v}_1 \cdot \vec{v}_2 \vec{v}_1 \cdot \vec{a}_2 - \frac{1}{2} \hat{n} \times \vec{S}_1 \cdot \vec{v}_1 \hat{n} \cdot \vec{v}_2 \vec{v}_1 \cdot \vec{a}_2 + \frac{1}{8} \vec{S}_1 \times \vec{v}_1 \cdot \vec{v}_2 \vec{v}_1 \cdot \vec{v}_1 - \frac{1}{6} \vec{S}_1 \times \vec{a}_1 \cdot \vec{v}_2 \vec{v}_1 \cdot \vec{v}_1 + \\
& \frac{3}{16} \vec{S}_1 \times \vec{v}_1 \cdot \vec{a}_1 \vec{v}_1 \cdot \vec{v}_1 + \frac{11}{48} \vec{S}_1 \times \vec{v}_1 \cdot \vec{a}_2 \vec{v}_1 \cdot \vec{v}_1 - \frac{11}{8} \hat{n} \times \vec{S}_1 \cdot \vec{v}_1 \hat{n} \cdot \vec{a}_1 \vec{v}_1 \cdot \vec{v}_1 - \frac{11}{24} \hat{n} \times \vec{S}_1 \cdot \vec{v}_1 \hat{n} \cdot \vec{a}_2 \vec{v}_1 \cdot \vec{v}_1 - \\
& \frac{1}{4} \hat{n} \times \vec{S}_1 \cdot \vec{v}_1 \hat{n} \cdot \vec{v}_2 \vec{v}_1 \cdot \vec{v}_1 + \frac{1}{3} \hat{n} \times \vec{S}_1 \cdot \vec{a}_1 \hat{n} \cdot \vec{v}_2 \vec{v}_1 \cdot \vec{v}_1 - \frac{2}{3} \vec{S}_1 \times \vec{v}_1 \cdot \vec{v}_2 \vec{v}_1 \cdot \vec{v}_2 - \frac{1}{4} \vec{S}_1 \times \vec{a}_1 \cdot \vec{v}_2 \vec{v}_1 \cdot \vec{v}_2 + \\
& \frac{1}{3} \vec{S}_1 \times \vec{v}_1 \cdot \vec{a}_1 \vec{v}_1 \cdot \vec{v}_2 + \frac{1}{4} \vec{S}_1 \times \vec{v}_1 \cdot \vec{a}_2 \vec{v}_1 \cdot \vec{v}_2 - \frac{1}{2} \hat{n} \times \vec{S}_1 \cdot \vec{v}_1 \hat{n} \cdot \vec{a}_2 \vec{v}_1 \cdot \vec{v}_2 + \frac{4}{3} \hat{n} \times \vec{S}_1 \cdot \vec{v}_1 \hat{n} \cdot \vec{v}_2 \vec{v}_1 \cdot \vec{v}_2 + \\
& \frac{1}{2} \hat{n} \times \vec{S}_1 \cdot \vec{a}_1 \hat{n} \cdot \vec{v}_2 \vec{v}_1 \cdot \vec{v}_2 + \frac{1}{2} \vec{S}_1 \times \vec{v}_1 \cdot \vec{v}_2 \vec{v}_2 \cdot \vec{v}_2 + \frac{1}{4} \vec{S}_1 \times \vec{a}_1 \cdot \vec{v}_2 \vec{v}_2 \cdot \vec{v}_2 + \frac{1}{12} \vec{S}_1 \times \vec{v}_1 \cdot \vec{a}_1 \vec{v}_2 \cdot \vec{v}_2 + \\
& \frac{1}{12} \hat{n} \times \vec{S}_1 \cdot \vec{v}_1 \hat{n} \cdot \vec{a}_1 \vec{v}_2 \cdot \vec{v}_2 - \hat{n} \times \vec{S}_1 \cdot \vec{v}_1 \hat{n} \cdot \vec{v}_2 \vec{v}_2 \cdot \vec{v}_2 - \frac{1}{2} \hat{n} \times \vec{S}_1 \cdot \vec{a}_1 \hat{n} \cdot \vec{v}_2 \vec{v}_2 \cdot \vec{v}_2 \Big) m_1 m_2 G^2 + \frac{1}{r^3} \\
& \left( \frac{55}{32} \hat{n} \times \vec{S}_1 \cdot \vec{v}_1 (\hat{n} \cdot \vec{v}_1)^4 + \frac{1}{3} \vec{S}_1 \times \vec{v}_1 \cdot \vec{v}_2 (\hat{n} \cdot \vec{v}_1)^3 - 2 \hat{n} \times \vec{S}_1 \cdot \vec{v}_1 \hat{n} \cdot \vec{v}_2 (\hat{n} \cdot \vec{v}_1)^3 - \frac{5}{2} \hat{n} \times \vec{S}_1 \cdot \vec{v}_1 (\hat{n} \cdot \vec{v}_2)^2 (\hat{n} \cdot \vec{v}_1)^2 + \right. \\
& \frac{5}{6} \vec{S}_1 \times \vec{v}_1 \cdot \vec{v}_2 \hat{n} \cdot \vec{v}_2 (\hat{n} \cdot \vec{v}_1)^2 + \frac{31}{16} \hat{n} \times \vec{S}_1 \cdot \vec{v}_1 \vec{v}_1 \cdot \vec{v}_1 (\hat{n} \cdot \vec{v}_1)^2 + \hat{n} \times \vec{S}_1 \cdot \vec{v}_1 \vec{v}_1 \cdot \vec{v}_2 (\hat{n} \cdot \vec{v}_1)^2 + \\
& \frac{5}{12} \hat{n} \times \vec{S}_1 \cdot \vec{v}_1 \vec{v}_2 \cdot \vec{v}_2 (\hat{n} \cdot \vec{v}_1)^2 + 4 \hat{n} \times \vec{S}_1 \cdot \vec{v}_1 (\hat{n} \cdot \vec{v}_2)^3 \hat{n} \cdot \vec{v}_1 - 2 \vec{S}_1 \times \vec{v}_1 \cdot \vec{v}_2 (\hat{n} \cdot \vec{v}_2)^2 \hat{n} \cdot \vec{v}_1 + \\
& \frac{1}{2} \vec{S}_1 \times \vec{v}_1 \cdot \vec{v}_2 \vec{v}_1 \cdot \vec{v}_1 \hat{n} \cdot \vec{v}_1 - 2 \hat{n} \times \vec{S}_1 \cdot \vec{v}_1 \hat{n} \cdot \vec{v}_2 \vec{v}_1 \cdot \vec{v}_1 \hat{n} \cdot \vec{v}_1 - \frac{5}{12} \vec{S}_1 \times \vec{v}_1 \cdot \vec{v}_2 \vec{v}_1 \cdot \vec{v}_2 \hat{n} \cdot \vec{v}_1 + \\
& \frac{5}{3} \hat{n} \times \vec{S}_1 \cdot \vec{v}_1 \hat{n} \cdot \vec{v}_2 \vec{v}_1 \cdot \vec{v}_2 \hat{n} \cdot \vec{v}_1 + \frac{1}{2} \vec{S}_1 \times \vec{v}_1 \cdot \vec{v}_2 \vec{v}_2 \cdot \vec{v}_2 \hat{n} \cdot \vec{v}_1 - 2 \hat{n} \times \vec{S}_1 \cdot \vec{v}_1 \hat{n} \cdot \vec{v}_2 \vec{v}_2 \cdot \vec{v}_2 \hat{n} \cdot \vec{v}_1 - \\
& \frac{13}{32} \hat{n} \times \vec{S}_1 \cdot \vec{v}_1 (\vec{v}_1 \cdot \vec{v}_1)^2 - \frac{5}{24} \hat{n} \times \vec{S}_1 \cdot \vec{v}_1 (\vec{v}_1 \cdot \vec{v}_2)^2 - \frac{11}{6} \hat{n} \times \vec{S}_1 \cdot \vec{v}_1 (\hat{n} \cdot \vec{v}_2)^2 \vec{v}_1 \cdot \vec{v}_1 + \\
& \frac{11}{12} \vec{S}_1 \times \vec{v}_1 \cdot \vec{v}_2 \hat{n} \cdot \vec{v}_2 \vec{v}_1 \cdot \vec{v}_1 - 2 \hat{n} \times \vec{S}_1 \cdot \vec{v}_1 (\hat{n} \cdot \vec{v}_2)^2 \vec{v}_1 \cdot \vec{v}_2 + \vec{S}_1 \times \vec{v}_1 \cdot \vec{v}_2 \hat{n} \cdot \vec{v}_2 \vec{v}_1 \cdot \vec{v}_2 + \\
& \left. \frac{1}{2} \hat{n} \times \vec{S}_1 \cdot \vec{v}_1 \vec{v}_1 \cdot \vec{v}_1 \vec{v}_1 \cdot \vec{v}_2 + \frac{11}{24} \hat{n} \times \vec{S}_1 \cdot \vec{v}_1 \vec{v}_1 \cdot \vec{v}_1 \vec{v}_2 \cdot \vec{v}_2 + \frac{1}{2} \hat{n} \times \vec{S}_1 \cdot \vec{v}_1 \vec{v}_1 \cdot \vec{v}_2 \vec{v}_2 \cdot \vec{v}_2 \right) m_1 m_2 G^2 + \\
& r m_1 m_2 \left( -\frac{1}{12} \log\left(\frac{r}{R_\theta}\right) \hat{n} \times \vec{S}_1 \cdot \vec{a}_1 + \frac{\frac{2}{24} \frac{1}{\vec{S}_1 \cdot \vec{a}_1}}{\epsilon_d} + \frac{17}{144} \hat{n} \times \vec{S}_1 \cdot \vec{a}_1 \right) G^2 + \\
& m_1 m_2 \left( \frac{1}{6} \log\left(\frac{r}{R_\theta}\right) \vec{S}_1 \times \vec{v}_1 \cdot \vec{a}_1 - \frac{17}{72} \vec{S}_1 \times \vec{v}_1 \cdot \vec{a}_1 - \frac{17}{72} \vec{S}_1 \times \vec{v}_1 \cdot \vec{a}_2 - \frac{17}{144} \vec{S}_1 \times \vec{a}_1 \cdot \vec{v}_2 + \frac{17}{144} \vec{S}_1 \times \vec{v}_1 \cdot \vec{a}_2 - \right. \\
& \frac{17}{144} \vec{S}_1 \times \vec{a}_1 \cdot \vec{a}_1 - \frac{17}{144} \vec{S}_1 \times \vec{a}_1 \cdot \vec{a}_2 + \frac{1}{4} \hat{n} \times \vec{S}_1 \cdot \vec{v}_1 \hat{n} \cdot \vec{a}_1 + \frac{1}{8} \hat{n} \times \vec{S}_1 \cdot \vec{a}_1 \hat{n} \cdot \vec{a}_1 + \frac{1}{6} \hat{n} \times \vec{S}_1 \cdot \vec{v}_1 \hat{n} \cdot \vec{a}_2 + \\
& \frac{1}{12} \hat{n} \times \vec{S}_1 \cdot \vec{a}_1 \hat{n} \cdot \vec{a}_2 - \frac{3}{8} \hat{n} \times \vec{S}_1 \cdot \vec{v}_1 \hat{n} \cdot \vec{a}_1 + \frac{1}{24} \hat{n} \times \vec{S}_1 \cdot \vec{a}_1 \hat{n} \cdot \vec{a}_1 - \frac{1}{12} \hat{n} \times \vec{S}_1 \cdot \vec{v}_1 \hat{n} \cdot \vec{a}_2 + \frac{1}{12} \hat{n} \times \vec{S}_1 \cdot \vec{a}_1 \hat{n} \cdot \vec{v}_1 - \\
& \frac{3}{8} \hat{n} \times \vec{S}_1 \cdot \vec{a}_1 \hat{n} \cdot \vec{v}_1 + \frac{1}{12} \hat{n} \times \vec{S}_1 \cdot \vec{a}_1 \hat{n} \cdot \vec{v}_2 + \frac{1}{6} \vec{S}_1 \times \vec{v}_1 \cdot \vec{a}_2 \log\left(\frac{r}{R_\theta}\right) + \frac{1}{12} \vec{S}_1 \times \vec{a}_1 \cdot \vec{v}_2 \log\left(\frac{r}{R_\theta}\right) - \\
& \frac{1}{12} \vec{S}_1 \times \vec{v}_1 \cdot \vec{a}_2 \log\left(\frac{r}{R_\theta}\right) + \frac{1}{12} \vec{S}_1 \times \vec{a}_1 \cdot \vec{a}_1 \log\left(\frac{r}{R_\theta}\right) + \frac{1}{12} \vec{S}_1 \times \vec{a}_1 \cdot \vec{a}_2 \log\left(\frac{r}{R_\theta}\right) + \frac{1}{\epsilon_d} \\
& \left. \left( -\frac{1}{12} \vec{S}_1 \times \vec{v}_1 \cdot \vec{a}_1 - \frac{1}{12} \vec{S}_1 \times \vec{v}_1 \cdot \vec{a}_2 - \frac{1}{24} \vec{S}_1 \times \vec{a}_1 \cdot \vec{v}_2 + \frac{1}{24} \vec{S}_1 \times \vec{v}_1 \cdot \vec{a}_2 - \frac{1}{24} \vec{S}_1 \times \vec{a}_1 \cdot \vec{a}_1 - \frac{1}{24} \vec{S}_1 \times \vec{a}_1 \cdot \vec{a}_2 \right) \right) G^2 \Big\}
\end{aligned}$$

{DiagSet[2, 2, 159],

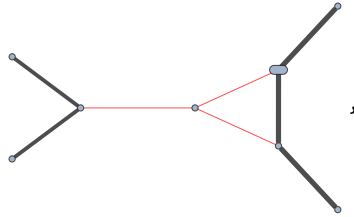

,

$$\frac{1}{r} \left( -4 \vec{S}_1 \times \vec{v}_1 \cdot \vec{a}_1 \hat{n} \cdot \vec{v}_1 - 4 \vec{S}_1 \times \vec{v}_1 \cdot \vec{a}_1 \hat{n} \cdot \vec{v}_1 + 8 \vec{S}_1 \times \vec{v}_1 \cdot \vec{a}_1 \hat{n} \cdot \vec{v}_2 + 8 \vec{S}_1 \times \vec{v}_1 \cdot \vec{a}_1 \hat{n} \cdot \vec{v}_2 + \right. \\ \left. 12 \hat{n} \times \vec{S}_1 \cdot \vec{v}_1 \vec{v}_1 \cdot \vec{a}_1 + 12 \hat{n} \times \vec{S}_1 \cdot \vec{a}_1 \vec{v}_1 \cdot \vec{a}_1 + 12 \hat{n} \times \vec{S}_1 \cdot \vec{v}_1 \vec{v}_2 \cdot \vec{a}_2 + 12 \hat{n} \times \vec{S}_1 \cdot \vec{a}_1 \vec{v}_2 \cdot \vec{a}_2 \right) m_1 m_2 G^2 + \frac{1}{r^2} \\ \left( 2 \vec{S}_1 \times \vec{v}_1 \cdot \vec{a}_1 (\hat{n} \cdot \vec{v}_1)^2 - 16 \vec{S}_1 \times \vec{v}_1 \cdot \vec{a}_1 \hat{n} \cdot \vec{v}_2 \hat{n} \cdot \vec{v}_1 - 20 \hat{n} \times \vec{S}_1 \cdot \vec{v}_1 \vec{v}_1 \cdot \vec{a}_1 \hat{n} \cdot \vec{v}_1 - 4 \hat{n} \times \vec{S}_1 \cdot \vec{v}_1 \vec{v}_1 \cdot \vec{v}_1 \hat{n} \cdot \vec{v}_1 - \right. \\ \left. 4 \hat{n} \times \vec{S}_1 \cdot \vec{a}_1 \vec{v}_1 \cdot \vec{v}_1 \hat{n} \cdot \vec{v}_1 - 24 \hat{n} \times \vec{S}_1 \cdot \vec{v}_1 \vec{v}_2 \cdot \vec{a}_2 \hat{n} \cdot \vec{v}_1 - 3 \hat{n} \times \vec{S}_1 \cdot \vec{v}_1 \vec{v}_2 \cdot \vec{v}_2 \hat{n} \cdot \vec{v}_1 - 3 \hat{n} \times \vec{S}_1 \cdot \vec{a}_1 \vec{v}_2 \cdot \vec{v}_2 \hat{n} \cdot \vec{v}_1 - \right. \\ \left. 16 \vec{S}_1 \times \vec{v}_1 \cdot \vec{v}_2 \vec{v}_1 \cdot \vec{a}_1 + 32 \hat{n} \times \vec{S}_1 \cdot \vec{v}_1 \hat{n} \cdot \vec{v}_2 \vec{v}_1 \cdot \vec{a}_1 - 8 \vec{S}_1 \times \vec{v}_1 \cdot \vec{v}_2 \vec{v}_1 \cdot \vec{v}_1 - 8 \vec{S}_1 \times \vec{a}_1 \cdot \vec{v}_2 \vec{v}_1 \cdot \vec{v}_1 - 6 \vec{S}_1 \times \vec{v}_1 \cdot \vec{a}_1 \vec{v}_1 \cdot \vec{v}_1 + \right. \\ \left. 16 \hat{n} \times \vec{S}_1 \cdot \vec{v}_1 \hat{n} \cdot \vec{v}_2 \vec{v}_1 \cdot \vec{v}_1 + 16 \hat{n} \times \vec{S}_1 \cdot \vec{a}_1 \hat{n} \cdot \vec{v}_2 \vec{v}_1 \cdot \vec{v}_1 + 8 \vec{S}_1 \times \vec{v}_1 \cdot \vec{a}_1 \vec{v}_1 \cdot \vec{v}_2 - 6 \vec{S}_1 \times \vec{v}_1 \cdot \vec{v}_2 \vec{v}_2 \cdot \vec{v}_2 - \right. \\ \left. 6 \vec{S}_1 \times \vec{a}_1 \cdot \vec{v}_2 \vec{v}_2 \cdot \vec{v}_2 - 3 \vec{S}_1 \times \vec{v}_1 \cdot \vec{a}_1 \vec{v}_2 \cdot \vec{v}_2 + 12 \hat{n} \times \vec{S}_1 \cdot \vec{v}_1 \hat{n} \cdot \vec{v}_2 \vec{v}_2 \cdot \vec{v}_2 + 12 \hat{n} \times \vec{S}_1 \cdot \vec{a}_1 \hat{n} \cdot \vec{v}_2 \vec{v}_2 \cdot \vec{v}_2 \right) m_1 m_2 G^2 + \\ \frac{1}{r^3} \left( 8 \hat{n} \times \vec{S}_1 \cdot \vec{v}_1 \vec{v}_1 \cdot \vec{v}_1 (\hat{n} \cdot \vec{v}_1)^2 + 6 \hat{n} \times \vec{S}_1 \cdot \vec{v}_1 \vec{v}_2 \cdot \vec{v}_2 (\hat{n} \cdot \vec{v}_1)^2 + 16 \vec{S}_1 \times \vec{v}_1 \cdot \vec{v}_2 \vec{v}_1 \cdot \vec{v}_1 \hat{n} \cdot \vec{v}_1 - 64 \hat{n} \times \vec{S}_1 \cdot \vec{v}_1 \right. \\ \left. \hat{n} \cdot \vec{v}_2 \vec{v}_1 \cdot \vec{v}_1 \hat{n} \cdot \vec{v}_1 + 12 \vec{S}_1 \times \vec{v}_1 \cdot \vec{v}_2 \vec{v}_2 \cdot \vec{v}_2 \hat{n} \cdot \vec{v}_1 - 48 \hat{n} \times \vec{S}_1 \cdot \vec{v}_1 \hat{n} \cdot \vec{v}_2 \vec{v}_2 \cdot \vec{v}_2 \hat{n} \cdot \vec{v}_1 - 4 \hat{n} \times \vec{S}_1 \cdot \vec{v}_1 (\vec{v}_1 \cdot \vec{v}_1)^2 + \right. \\ \left. 16 \hat{n} \times \vec{S}_1 \cdot \vec{v}_1 \vec{v}_1 \cdot \vec{v}_1 \vec{v}_1 \cdot \vec{v}_2 - 3 \hat{n} \times \vec{S}_1 \cdot \vec{v}_1 \vec{v}_1 \cdot \vec{v}_1 \vec{v}_2 \cdot \vec{v}_2 + 12 \hat{n} \times \vec{S}_1 \cdot \vec{v}_1 \vec{v}_1 \cdot \vec{v}_2 \vec{v}_2 \cdot \vec{v}_2 \right) m_1 m_2 G^2 \Big\}$$

{DiagSet[2, 2, 160],

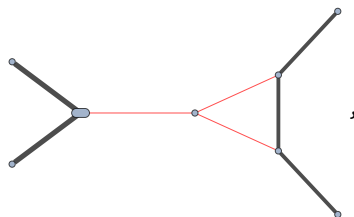

,

$$\frac{1}{r} G^2 \left( 4 \vec{a}_1 \times \vec{S}_1 \cdot \vec{v}_1 \hat{n} \cdot \vec{v}_2 + 4 \vec{a}_1 \times \vec{S}_1 \cdot \vec{v}_1 \hat{n} \cdot \vec{v}_2 + 24 \hat{n} \times \vec{S}_1 \cdot \vec{v}_1 \vec{a}_2 \cdot \vec{v}_2 - 24 \hat{n} \times \vec{a}_1 \cdot \vec{S}_1 \vec{a}_2 \cdot \vec{v}_2 \right) m_2^2 + \frac{1}{r^2} \\ G^2 \left( \vec{a}_1 \times \vec{S}_1 \cdot \vec{v}_1 (\hat{n} \cdot \vec{v}_2)^2 - 8 \vec{a}_1 \times \vec{S}_1 \cdot \vec{v}_1 \hat{n} \cdot \vec{v}_1 \hat{n} \cdot \vec{v}_2 + 8 \hat{n} \times \vec{S}_1 \cdot \vec{v}_1 \vec{a}_1 \cdot \vec{v}_1 \hat{n} \cdot \vec{v}_2 + 24 \hat{n} \times \vec{S}_1 \cdot \vec{v}_1 \vec{a}_2 \cdot \vec{v}_2 \hat{n} \cdot \vec{v}_2 + \right. \\ \left. 4 \hat{n} \times \vec{S}_1 \cdot \vec{v}_1 \vec{v}_1 \cdot \vec{v}_1 \hat{n} \cdot \vec{v}_2 - 4 \hat{n} \times \vec{a}_1 \cdot \vec{S}_1 \vec{v}_1 \cdot \vec{v}_1 \hat{n} \cdot \vec{v}_2 + 24 \hat{n} \times \vec{S}_1 \cdot \vec{v}_1 \vec{v}_2 \cdot \vec{v}_2 \hat{n} \cdot \vec{v}_2 - 24 \hat{n} \times \vec{a}_1 \cdot \vec{S}_1 \vec{v}_2 \cdot \vec{v}_2 \hat{n} \cdot \vec{v}_2 - \right. \\ \left. 4 \vec{S}_1 \times \vec{v}_1 \cdot \vec{v}_2 \vec{a}_1 \cdot \vec{v}_1 - 12 \vec{S}_1 \times \vec{v}_1 \cdot \vec{v}_2 \vec{a}_2 \cdot \vec{v}_2 - 48 \hat{n} \times \vec{S}_1 \cdot \vec{v}_1 \hat{n} \cdot \vec{v}_1 \vec{a}_2 \cdot \vec{v}_2 - 2 \vec{S}_1 \times \vec{v}_1 \cdot \vec{v}_2 \vec{v}_1 \cdot \vec{v}_1 + \right. \\ \left. 2 \vec{a}_1 \times \vec{S}_1 \cdot \vec{v}_2 \vec{v}_1 \cdot \vec{v}_1 + 4 \vec{a}_1 \times \vec{S}_1 \cdot \vec{v}_1 \vec{v}_1 \cdot \vec{v}_2 - 12 \vec{S}_1 \times \vec{v}_1 \cdot \vec{v}_2 \vec{v}_2 \cdot \vec{v}_2 - \vec{a}_1 \times \vec{S}_1 \cdot \vec{v}_1 \vec{v}_2 \cdot \vec{v}_2 + 12 \vec{a}_1 \times \vec{S}_1 \cdot \vec{v}_2 \vec{v}_2 \cdot \vec{v}_2 \right) m_2^2 + \\ \frac{1}{r^3} G^2 \left( 2 \hat{n} \times \vec{S}_1 \cdot \vec{v}_1 \vec{v}_1 \cdot \vec{v}_1 (\hat{n} \cdot \vec{v}_2)^2 + 12 \hat{n} \times \vec{S}_1 \cdot \vec{v}_1 \vec{v}_2 \cdot \vec{v}_2 (\hat{n} \cdot \vec{v}_2)^2 - \vec{S}_1 \times \vec{v}_1 \cdot \vec{v}_2 \vec{v}_1 \cdot \vec{v}_1 \hat{n} \cdot \vec{v}_2 - \right. \\ \left. 16 \hat{n} \times \vec{S}_1 \cdot \vec{v}_1 \hat{n} \cdot \vec{v}_1 \vec{v}_1 \cdot \vec{v}_1 \hat{n} \cdot \vec{v}_2 - 6 \vec{S}_1 \times \vec{v}_1 \cdot \vec{v}_2 \vec{v}_2 \cdot \vec{v}_2 \hat{n} \cdot \vec{v}_2 - 96 \hat{n} \times \vec{S}_1 \cdot \vec{v}_1 \hat{n} \cdot \vec{v}_1 \vec{v}_2 \cdot \vec{v}_2 \hat{n} \cdot \vec{v}_2 - \right. \\ \left. 6 \hat{n} \times \vec{S}_1 \cdot \vec{v}_1 (\vec{v}_2 \cdot \vec{v}_2)^2 + 4 \vec{S}_1 \times \vec{v}_1 \cdot \vec{v}_2 \hat{n} \cdot \vec{v}_1 \vec{v}_1 \cdot \vec{v}_1 + 4 \hat{n} \times \vec{S}_1 \cdot \vec{v}_1 \vec{v}_1 \cdot \vec{v}_1 \vec{v}_1 \cdot \vec{v}_2 + \right. \\ \left. 24 \vec{S}_1 \times \vec{v}_1 \cdot \vec{v}_2 \hat{n} \cdot \vec{v}_1 \vec{v}_2 \cdot \vec{v}_2 - \hat{n} \times \vec{S}_1 \cdot \vec{v}_1 \vec{v}_1 \cdot \vec{v}_1 \vec{v}_2 \cdot \vec{v}_2 + 24 \hat{n} \times \vec{S}_1 \cdot \vec{v}_1 \vec{v}_1 \cdot \vec{v}_2 \vec{v}_2 \cdot \vec{v}_2 \right) m_2^2 \Big\}$$

{DiagSet[2, 2, 161],

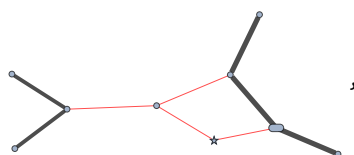

,



[illegible]

$$\begin{aligned}
& \frac{64}{3} \hat{n} \times \vec{S}_1 \cdot \vec{v}_1 \hat{n} \cdot \vec{v}_2 \vec{v}_1 \cdot \vec{v}_2 \hat{n} \cdot \vec{v}_1 - \frac{1}{2} \hat{n} \times \vec{S}_1 \cdot \vec{v}_1 (\vec{v}_1 \cdot \vec{v}_1)^2 + \frac{8}{3} \hat{n} \times \vec{S}_1 \cdot \vec{v}_1 (\vec{v}_1 \cdot \vec{v}_2)^2 - \\
& \frac{16}{3} \hat{n} \times \vec{S}_1 \cdot \vec{v}_1 (\hat{n} \cdot \vec{v}_2)^2 \vec{v}_1 \cdot \vec{v}_1 + \frac{8}{3} \vec{S}_1 \times \vec{v}_1 \cdot \vec{v}_2 \hat{n} \cdot \vec{v}_2 \vec{v}_1 \cdot \vec{v}_1 + \frac{4}{3} \hat{n} \times \vec{S}_1 \cdot \vec{v}_1 \vec{v}_1 \cdot \vec{v}_1 \vec{v}_2 \cdot \vec{v}_2 \Big) m_1 m_2 G^2 + \\
& m_1 m_2 \left( \frac{8}{3} \log\left(\frac{r}{R_0}\right) \frac{1}{\vec{S}_1 \times \vec{a}_1 \cdot \vec{a}_2} - \frac{4}{9} \frac{1}{\vec{S}_1 \times \vec{a}_1 \cdot \vec{a}_2} - \frac{8}{9} \frac{2}{\vec{S}_1 \times \vec{v}_1 \cdot \vec{a}_1} - \frac{2}{9} \frac{2}{\vec{S}_1 \times \vec{v}_1 \cdot \vec{a}_2} - \frac{2}{9} \frac{1}{\vec{S}_1 \times \vec{a}_1 \cdot \vec{a}_2} + \frac{8}{9} \frac{1}{\vec{S}_1 \times \vec{a}_1 \cdot \vec{a}_1} - \right. \\
& \frac{4}{3} \hat{n} \times \vec{S}_1 \cdot \vec{a}_1 \hat{n} \cdot \vec{a}_1 - \frac{2}{3} \hat{n} \times \vec{S}_1 \cdot \vec{v}_1 \hat{n} \cdot \vec{a}_1 - \frac{2}{3} \hat{n} \times \vec{S}_1 \cdot \vec{a}_1 \hat{n} \cdot \vec{a}_1 + \frac{8}{3} \hat{n} \times \vec{S}_1 \cdot \vec{a}_1 \hat{n} \cdot \vec{a}_2 + \frac{4}{3} \hat{n} \times \vec{S}_1 \cdot \vec{v}_1 \hat{n} \cdot \vec{a}_2 + \\
& \frac{4}{3} \hat{n} \times \vec{S}_1 \cdot \vec{a}_1 \hat{n} \cdot \vec{a}_2 + \frac{4}{3} \frac{2}{\vec{S}_1 \times \vec{v}_1 \cdot \vec{a}_1} \log\left(\frac{r}{R_0}\right) + \frac{4}{3} \frac{2}{\vec{S}_1 \times \vec{v}_1 \cdot \vec{a}_2} \log\left(\frac{r}{R_0}\right) + \frac{4}{3} \frac{1}{\vec{S}_1 \times \vec{a}_1 \cdot \vec{a}_2} \log\left(\frac{r}{R_0}\right) - \\
& \left. \frac{4}{3} \frac{1}{\vec{S}_1 \times \vec{a}_1 \cdot \vec{a}_1} \log\left(\frac{r}{R_0}\right) + \frac{-\frac{4}{3} \frac{1}{\vec{S}_1 \times \vec{a}_1 \cdot \vec{a}_2} - \frac{2}{3} \frac{2}{\vec{S}_1 \times \vec{v}_1 \cdot \vec{a}_1} - \frac{2}{3} \frac{2}{\vec{S}_1 \times \vec{v}_1 \cdot \vec{a}_2} - \frac{2}{3} \frac{1}{\vec{S}_1 \times \vec{a}_1 \cdot \vec{a}_2} + \frac{2}{3} \frac{1}{\vec{S}_1 \times \vec{a}_1 \cdot \vec{a}_1}}{\epsilon_d} \right) G^2 \Big\}
\end{aligned}$$

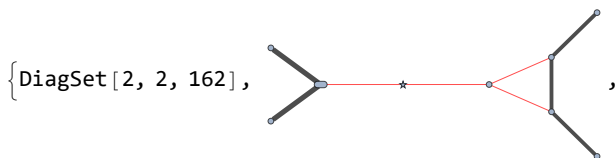

$$\begin{aligned}
& \frac{1}{r} G^2 \left( -\frac{8}{3} \hat{n} \times \vec{a}_1 \cdot \vec{S}_1 (\hat{n} \cdot \vec{v}_2)^2 + \frac{8}{3} \hat{n} \times \vec{S}_1 \cdot \vec{v}_1 (\hat{n} \cdot \vec{v}_2)^2 - \frac{16}{3} \hat{n} \times \vec{a}_1 \cdot \vec{S}_1 (\hat{n} \cdot \vec{v}_2)^2 + \frac{8}{3} \frac{1}{\vec{a}_1 \times \vec{S}_1 \cdot \vec{v}_2} \hat{n} \cdot \vec{v}_2 - \right. \\
& \frac{8}{3} \frac{2}{\vec{S}_1 \times \vec{v}_1 \cdot \vec{v}_2} \hat{n} \cdot \vec{v}_2 + \frac{16}{3} \vec{a}_1 \times \vec{S}_1 \cdot \vec{v}_2 \hat{n} \cdot \vec{v}_2 - \frac{1}{3} \vec{a}_1 \times \vec{a}_2 \cdot \vec{S}_1 \hat{n} \cdot \vec{v}_2 - \frac{1}{3} \vec{a}_2 \times \vec{S}_1 \cdot \vec{v}_1 \hat{n} \cdot \vec{v}_2 + \frac{2}{3} \hat{n} \times \vec{S}_1 \cdot \vec{v}_1 \hat{n} \cdot \vec{a}_2 \hat{n} \cdot \vec{v}_2 - \\
& \frac{2}{3} \hat{n} \times \vec{a}_1 \cdot \vec{S}_1 \hat{n} \cdot \vec{a}_2 \hat{n} \cdot \vec{v}_2 + \frac{4}{3} \vec{a}_2 \times \vec{S}_1 \cdot \vec{v}_1 \hat{n} \cdot \vec{a}_1 - \frac{1}{3} \frac{1}{\vec{S}_1 \times \vec{v}_1 \cdot \vec{v}_2} \hat{n} \cdot \vec{a}_2 - \frac{4}{3} \vec{a}_1 \times \vec{S}_1 \cdot \vec{v}_1 \hat{n} \cdot \vec{a}_2 + \frac{1}{3} \vec{a}_1 \times \vec{S}_1 \cdot \vec{v}_2 \hat{n} \cdot \vec{a}_2 - \\
& \frac{8}{3} \hat{n} \times \vec{S}_1 \cdot \vec{v}_1 \hat{n} \cdot \vec{a}_1 \hat{n} \cdot \vec{a}_2 + \frac{8}{3} \vec{a}_1 \times \vec{a}_2 \cdot \vec{S}_1 \hat{n} \cdot \vec{v}_1 + \frac{8}{3} \vec{a}_2 \times \vec{S}_1 \cdot \vec{v}_1 \hat{n} \cdot \vec{v}_1 - \frac{16}{3} \hat{n} \times \vec{S}_1 \cdot \vec{v}_1 \hat{n} \cdot \vec{a}_2 \hat{n} \cdot \vec{v}_1 + \\
& \frac{16}{3} \hat{n} \times \vec{a}_1 \cdot \vec{S}_1 \hat{n} \cdot \vec{a}_2 \hat{n} \cdot \vec{v}_1 + \frac{4}{3} \hat{n} \times \vec{S}_1 \cdot \vec{v}_1 \vec{a}_1 \cdot \vec{a}_2 + \frac{8}{3} \hat{n} \times \vec{S}_1 \cdot \vec{v}_1 \vec{a}_2 \cdot \vec{v}_1 - \frac{8}{3} \hat{n} \times \vec{a}_1 \cdot \vec{S}_1 \vec{a}_2 \cdot \vec{v}_1 - \\
& \frac{4}{3} \hat{n} \times \vec{S}_1 \cdot \vec{v}_1 \vec{a}_2 \cdot \vec{v}_2 + \frac{4}{3} \hat{n} \times \vec{a}_1 \cdot \vec{S}_1 \vec{a}_2 \cdot \vec{v}_2 + \frac{4}{3} \hat{n} \times \vec{a}_1 \cdot \vec{S}_1 \vec{v}_2 \cdot \vec{v}_2 - \frac{4}{3} \hat{n} \times \vec{S}_1 \cdot \vec{v}_1 \vec{v}_2 \cdot \vec{v}_2 + \frac{8}{3} \hat{n} \times \vec{a}_1 \cdot \vec{S}_1 \vec{v}_2 \cdot \vec{v}_2 \Big) m_2^2 + \\
& \frac{1}{r^2} G^2 \left( \frac{4}{3} \hat{n} \times \vec{S}_1 \cdot \vec{v}_1 (\hat{n} \cdot \vec{v}_2)^3 - \frac{4}{3} \hat{n} \times \vec{a}_1 \cdot \vec{S}_1 (\hat{n} \cdot \vec{v}_2)^3 - \frac{1}{\vec{S}_1 \times \vec{v}_1 \cdot \vec{v}_2} (\hat{n} \cdot \vec{v}_2)^2 - \frac{8}{3} \vec{a}_1 \times \vec{S}_1 \cdot \vec{v}_1 (\hat{n} \cdot \vec{v}_2)^2 + \right. \\
& \vec{a}_1 \times \vec{S}_1 \cdot \vec{v}_2 (\hat{n} \cdot \vec{v}_2)^2 - \frac{32}{3} \hat{n} \times \vec{S}_1 \cdot \vec{v}_1 \hat{n} \cdot \vec{a}_1 (\hat{n} \cdot \vec{v}_2)^2 - \frac{64}{3} \hat{n} \times \vec{S}_1 \cdot \vec{v}_1 \hat{n} \cdot \vec{v}_1 (\hat{n} \cdot \vec{v}_2)^2 + \frac{64}{3} \hat{n} \times \vec{a}_1 \cdot \vec{S}_1 \hat{n} \cdot \vec{v}_1 (\hat{n} \cdot \vec{v}_2)^2 + \\
& \frac{16}{3} \vec{S}_1 \times \vec{v}_1 \cdot \vec{v}_2 \hat{n} \cdot \vec{a}_1 \hat{n} \cdot \vec{v}_2 + \frac{32}{3} \frac{1}{\vec{S}_1 \times \vec{v}_1 \cdot \vec{v}_2} \hat{n} \cdot \vec{v}_1 \hat{n} \cdot \vec{v}_2 - \frac{32}{3} \vec{a}_1 \times \vec{S}_1 \cdot \vec{v}_2 \hat{n} \cdot \vec{v}_1 \hat{n} \cdot \vec{v}_2 + \frac{2}{3} \vec{a}_2 \times \vec{S}_1 \cdot \vec{v}_1 \hat{n} \cdot \vec{v}_1 \hat{n} \cdot \vec{v}_2 - \\
& \frac{8}{3} \hat{n} \times \vec{S}_1 \cdot \vec{v}_1 \hat{n} \cdot \vec{a}_2 \hat{n} \cdot \vec{v}_1 \hat{n} \cdot \vec{v}_2 + \frac{16}{3} \hat{n} \times \vec{S}_1 \cdot \vec{v}_1 \vec{a}_1 \cdot \vec{v}_2 \hat{n} \cdot \vec{v}_2 + \frac{2}{3} \hat{n} \times \vec{S}_1 \cdot \vec{v}_1 \vec{a}_2 \cdot \vec{v}_1 \hat{n} \cdot \vec{v}_2 + \\
& \frac{32}{3} \hat{n} \times \vec{S}_1 \cdot \vec{v}_1 \vec{v}_1 \cdot \vec{v}_2 \hat{n} \cdot \vec{v}_2 - \frac{32}{3} \hat{n} \times \vec{a}_1 \cdot \vec{S}_1 \vec{v}_1 \cdot \vec{v}_2 \hat{n} \cdot \vec{v}_2 - 2 \hat{n} \times \vec{S}_1 \cdot \vec{v}_1 \vec{v}_2 \cdot \vec{v}_2 \hat{n} \cdot \vec{v}_2 + 2 \hat{n} \times \vec{a}_1 \cdot \vec{S}_1 \vec{v}_2 \cdot \vec{v}_2 \hat{n} \cdot \vec{v}_2 - \\
& \frac{8}{3} \vec{a}_2 \times \vec{S}_1 \cdot \vec{v}_1 (\hat{n} \cdot \vec{v}_1)^2 + \frac{32}{3} \hat{n} \times \vec{S}_1 \cdot \vec{v}_1 \hat{n} \cdot \vec{a}_2 (\hat{n} \cdot \vec{v}_1)^2 + \frac{2}{3} \vec{S}_1 \times \vec{v}_1 \cdot \vec{v}_2 \hat{n} \cdot \vec{a}_2 \hat{n} \cdot \vec{v}_1 - \frac{8}{3} \vec{S}_1 \times \vec{v}_1 \cdot \vec{v}_2 \vec{a}_1 \cdot \vec{v}_2 - \\
& \frac{1}{3} \vec{S}_1 \times \vec{v}_1 \cdot \vec{v}_2 \vec{a}_2 \cdot \vec{v}_1 - \frac{16}{3} \hat{n} \times \vec{S}_1 \cdot \vec{v}_1 \hat{n} \cdot \vec{v}_1 \vec{a}_2 \cdot \vec{v}_1 + \frac{8}{3} \hat{n} \times \vec{S}_1 \cdot \vec{v}_1 \hat{n} \cdot \vec{v}_1 \vec{a}_2 \cdot \vec{v}_2 + \frac{4}{3} \vec{a}_2 \times \vec{S}_1 \cdot \vec{v}_1 \vec{v}_1 \cdot \vec{v}_1 - \\
& \frac{8}{3} \hat{n} \times \vec{S}_1 \cdot \vec{v}_1 \hat{n} \cdot \vec{a}_2 \vec{v}_1 \cdot \vec{v}_1 - \frac{16}{3} \frac{1}{\vec{S}_1 \times \vec{v}_1 \cdot \vec{v}_2} \vec{v}_1 \cdot \vec{v}_2 + \frac{16}{3} \vec{a}_1 \times \vec{S}_1 \cdot \vec{v}_2 \vec{v}_1 \cdot \vec{v}_2 - \frac{1}{3} \vec{a}_2 \times \vec{S}_1 \cdot \vec{v}_1 \vec{v}_1 \cdot \vec{v}_2 + \\
& \frac{2}{3} \hat{n} \times \vec{S}_1 \cdot \vec{v}_1 \hat{n} \cdot \vec{a}_2 \vec{v}_1 \cdot \vec{v}_2 + \frac{1}{\vec{S}_1 \times \vec{v}_1 \cdot \vec{v}_2} \vec{v}_2 \cdot \vec{v}_2 + \frac{4}{3} \vec{a}_1 \times \vec{S}_1 \cdot \vec{v}_1 \vec{v}_2 \cdot \vec{v}_2 - \vec{a}_1 \times \vec{S}_1 \cdot \vec{v}_2 \vec{v}_2 \cdot \vec{v}_2 +
\end{aligned}$$

$$\begin{aligned}
 & \frac{8}{3} \hat{n} \times \vec{S}_1 \cdot \vec{v}_1 \hat{n} \cdot \vec{a}_1 \vec{v}_2 \cdot \vec{v}_2 + \frac{16}{3} \hat{n} \times \vec{S}_1 \cdot \vec{v}_1 \hat{n} \cdot \vec{v}_1 \vec{v}_2 \cdot \vec{v}_2 - \frac{16}{3} \hat{n} \times \vec{a}_1 \cdot \vec{S}_1 \hat{n} \cdot \vec{v}_1 \vec{v}_2 \cdot \vec{v}_2 \Big) m_2^2 + \frac{1}{r^3} \\
 G^2 & \left( -8 \hat{n} \times \vec{S}_1 \cdot \vec{v}_1 \hat{n} \cdot \vec{v}_1 (\hat{n} \cdot \vec{v}_2)^3 + 64 \hat{n} \times \vec{S}_1 \cdot \vec{v}_1 (\hat{n} \cdot \vec{v}_1)^2 (\hat{n} \cdot \vec{v}_2)^2 + 4 \vec{S}_1 \times \vec{v}_1 \cdot \vec{v}_2 \hat{n} \cdot \vec{v}_1 (\hat{n} \cdot \vec{v}_2)^2 - \right. \\
 & \frac{32}{3} \hat{n} \times \vec{S}_1 \cdot \vec{v}_1 \vec{v}_1 \cdot \vec{v}_1 (\hat{n} \cdot \vec{v}_2)^2 + 4 \hat{n} \times \vec{S}_1 \cdot \vec{v}_1 \vec{v}_1 \cdot \vec{v}_2 (\hat{n} \cdot \vec{v}_2)^2 - \frac{64}{3} \vec{S}_1 \times \vec{v}_1 \cdot \vec{v}_2 (\hat{n} \cdot \vec{v}_1)^2 \hat{n} \cdot \vec{v}_2 + \\
 & \frac{16}{3} \vec{S}_1 \times \vec{v}_1 \cdot \vec{v}_2 \vec{v}_1 \cdot \vec{v}_1 \hat{n} \cdot \vec{v}_2 - 2 \vec{S}_1 \times \vec{v}_1 \cdot \vec{v}_2 \vec{v}_1 \cdot \vec{v}_2 \hat{n} \cdot \vec{v}_2 - \frac{128}{3} \hat{n} \times \vec{S}_1 \cdot \vec{v}_1 \hat{n} \cdot \vec{v}_1 \vec{v}_1 \cdot \vec{v}_2 \hat{n} \cdot \vec{v}_2 + \\
 & 8 \hat{n} \times \vec{S}_1 \cdot \vec{v}_1 \hat{n} \cdot \vec{v}_1 \vec{v}_2 \cdot \vec{v}_2 \hat{n} \cdot \vec{v}_2 + \frac{16}{3} \hat{n} \times \vec{S}_1 \cdot \vec{v}_1 (\vec{v}_1 \cdot \vec{v}_2)^2 + \frac{32}{3} \vec{S}_1 \times \vec{v}_1 \cdot \vec{v}_2 \hat{n} \cdot \vec{v}_1 \vec{v}_1 \cdot \vec{v}_2 - \\
 & \left. \frac{32}{3} \hat{n} \times \vec{S}_1 \cdot \vec{v}_1 (\hat{n} \cdot \vec{v}_1)^2 \vec{v}_2 \cdot \vec{v}_2 - 2 \vec{S}_1 \times \vec{v}_1 \cdot \vec{v}_2 \hat{n} \cdot \vec{v}_1 \vec{v}_2 \cdot \vec{v}_2 + \frac{8}{3} \hat{n} \times \vec{S}_1 \cdot \vec{v}_1 \vec{v}_1 \cdot \vec{v}_1 \vec{v}_2 \cdot \vec{v}_2 - 2 \hat{n} \times \vec{S}_1 \cdot \vec{v}_1 \vec{v}_1 \cdot \vec{v}_2 \vec{v}_2 \cdot \vec{v}_2 \right) \\
 m_2^2 + G^2 & \left( \frac{4}{3} \log \left( \frac{r}{R_\theta} \right) \frac{1}{\vec{a}_1 \times \vec{a}_2 \cdot \vec{S}_1} - \frac{8}{9} \frac{1}{\vec{a}_1 \times \vec{a}_2 \cdot \vec{S}_1} - \frac{16}{9} \vec{a}_1 \times \vec{a}_2 \cdot \frac{1}{\vec{S}_1} - \frac{8}{9} \vec{a}_2 \times \vec{S}_1 \cdot \frac{2}{\vec{v}_1} - \frac{4}{3} \hat{n} \times \frac{1}{\vec{a}_1} \cdot \vec{S}_1 \hat{n} \cdot \vec{a}_2 + \right. \\
 & \frac{4}{3} \hat{n} \times \frac{2}{\vec{S}_1} \cdot \vec{v}_1 \hat{n} \cdot \vec{a}_2 - \frac{8}{3} \hat{n} \times \vec{a}_1 \cdot \frac{1}{\vec{S}_1} \hat{n} \cdot \vec{a}_2 + \frac{8}{3} \vec{a}_1 \times \vec{a}_2 \cdot \frac{1}{\vec{S}_1} \log \left( \frac{r}{R_\theta} \right) + \\
 & \left. \frac{4}{3} \vec{a}_2 \times \frac{2}{\vec{S}_1} \cdot \vec{v}_1 \log \left( \frac{r}{R_\theta} \right) + \frac{-\frac{2}{3} \frac{1}{\vec{a}_1 \times \vec{a}_2 \cdot \vec{S}_1} - \frac{4}{3} \vec{a}_1 \times \vec{a}_2 \cdot \frac{1}{\vec{S}_1} - \frac{2}{3} \vec{a}_2 \times \frac{2}{\vec{S}_1} \cdot \vec{v}_1}{\epsilon_d} \right) m_2^2 \Big\}
 \end{aligned}$$

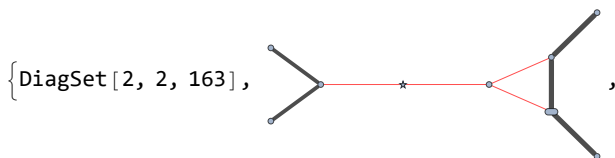

$$\begin{aligned}
 & \frac{1}{r} \left( \frac{16}{3} \hat{n} \times \vec{S}_1 \cdot \vec{a}_1 (\hat{n} \cdot \vec{v}_2)^2 + \frac{8}{3} \hat{n} \times \vec{S}_1 \cdot \vec{v}_1 (\hat{n} \cdot \vec{v}_2)^2 + \frac{8}{3} \hat{n} \times \vec{S}_1 \cdot \frac{1}{\vec{a}_1} (\hat{n} \cdot \vec{v}_2)^2 - \frac{16}{3} \vec{S}_1 \times \vec{a}_1 \cdot \vec{v}_2 \hat{n} \cdot \vec{v}_2 - \right. \\
 & \frac{4}{3} \vec{S}_1 \times \vec{v}_1 \cdot \vec{a}_1 \hat{n} \cdot \vec{v}_2 - \frac{8}{3} \vec{S}_1 \times \vec{v}_1 \cdot \vec{v}_2 \hat{n} \cdot \vec{v}_2 - \frac{8}{3} \vec{S}_1 \times \frac{1}{\vec{a}_1} \cdot \vec{v}_2 \hat{n} \cdot \vec{v}_2 - \frac{4}{3} \vec{S}_1 \times \vec{v}_1 \cdot \frac{1}{\vec{a}_1} \hat{n} \cdot \vec{v}_2 - \frac{2}{3} \hat{n} \times \frac{1}{\vec{S}_1} \cdot \vec{v}_1 \hat{n} \cdot \vec{a}_1 \hat{n} \cdot \vec{v}_2 - \\
 & \frac{2}{3} \hat{n} \times \vec{S}_1 \cdot \vec{a}_1 \hat{n} \cdot \vec{a}_1 \hat{n} \cdot \vec{v}_2 - \frac{4}{3} \hat{n} \times \vec{S}_1 \cdot \vec{a}_1 \hat{n} \cdot \vec{v}_1 \hat{n} \cdot \vec{v}_2 - \frac{2}{3} \hat{n} \times \vec{S}_1 \cdot \vec{v}_1 \hat{n} \cdot \vec{v}_1 \hat{n} \cdot \vec{v}_2 - \frac{2}{3} \hat{n} \times \vec{S}_1 \cdot \frac{1}{\vec{a}_1} \hat{n} \cdot \vec{v}_1 \hat{n} \cdot \vec{v}_2 + \\
 & \frac{1}{3} \vec{S}_1 \times \vec{v}_1 \cdot \vec{v}_2 \hat{n} \cdot \vec{a}_1 + \frac{1}{3} \vec{S}_1 \times \vec{a}_1 \cdot \vec{v}_2 \hat{n} \cdot \vec{a}_1 + \frac{4}{3} \vec{S}_1 \times \vec{v}_1 \cdot \vec{a}_2 \hat{n} \cdot \vec{a}_1 - \frac{4}{3} \vec{S}_1 \times \vec{v}_1 \cdot \vec{a}_1 \hat{n} \cdot \vec{a}_2 - \frac{8}{3} \hat{n} \times \vec{S}_1 \cdot \vec{v}_1 \hat{n} \cdot \vec{a}_1 \hat{n} \cdot \vec{a}_2 + \\
 & \frac{2}{3} \vec{S}_1 \times \vec{a}_1 \cdot \vec{v}_2 \hat{n} \cdot \vec{v}_1 + \frac{8}{3} \vec{S}_1 \times \vec{v}_1 \cdot \vec{a}_2 \hat{n} \cdot \vec{v}_1 + \frac{1}{3} \vec{S}_1 \times \vec{v}_1 \cdot \vec{v}_2 \hat{n} \cdot \vec{v}_1 + \frac{1}{3} \vec{S}_1 \times \frac{1}{\vec{a}_1} \cdot \vec{v}_2 \hat{n} \cdot \vec{v}_1 + \frac{8}{3} \vec{S}_1 \times \vec{a}_1 \cdot \vec{a}_2 \hat{n} \cdot \vec{v}_1 - \\
 & \frac{16}{3} \hat{n} \times \vec{S}_1 \cdot \vec{v}_1 \hat{n} \cdot \vec{a}_2 \hat{n} \cdot \vec{v}_1 - \frac{16}{3} \hat{n} \times \vec{S}_1 \cdot \vec{a}_1 \hat{n} \cdot \vec{a}_2 \hat{n} \cdot \vec{v}_1 + \frac{4}{3} \hat{n} \times \vec{S}_1 \cdot \vec{v}_1 \vec{a}_1 \cdot \vec{a}_2 + \frac{1}{3} \hat{n} \times \vec{S}_1 \cdot \vec{v}_1 \vec{a}_1 \cdot \vec{v}_2 + \\
 & \frac{1}{3} \hat{n} \times \vec{S}_1 \cdot \vec{a}_1 \vec{a}_1 \cdot \vec{v}_2 + \frac{8}{3} \hat{n} \times \vec{S}_1 \cdot \vec{v}_1 \vec{v}_1 \cdot \vec{a}_2 + \frac{8}{3} \hat{n} \times \vec{S}_1 \cdot \vec{a}_1 \vec{v}_1 \cdot \vec{a}_2 + \frac{2}{3} \hat{n} \times \vec{S}_1 \cdot \vec{a}_1 \vec{v}_1 \cdot \vec{v}_2 + \frac{1}{3} \hat{n} \times \vec{S}_1 \cdot \vec{v}_1 \vec{v}_1 \cdot \vec{v}_2 + \\
 & \left. \frac{1}{3} \hat{n} \times \vec{S}_1 \cdot \frac{1}{\vec{a}_1} \vec{v}_1 \cdot \vec{v}_2 - \frac{8}{3} \hat{n} \times \vec{S}_1 \cdot \vec{a}_1 \vec{v}_2 \cdot \vec{v}_2 - \frac{4}{3} \hat{n} \times \vec{S}_1 \cdot \vec{v}_1 \vec{v}_2 \cdot \vec{v}_2 - \frac{4}{3} \hat{n} \times \vec{S}_1 \cdot \frac{1}{\vec{a}_1} \vec{v}_2 \cdot \vec{v}_2 \right) m_1 m_2 G^2 + \frac{1}{r^2} \\
 & \left( - \left( \vec{S}_1 \times \vec{v}_1 \cdot \vec{v}_2 \right) (\hat{n} \cdot \vec{v}_1)^2 - \vec{S}_1 \times \vec{a}_1 \cdot \vec{v}_2 (\hat{n} \cdot \vec{v}_1)^2 - \frac{8}{3} \vec{S}_1 \times \vec{v}_1 \cdot \vec{a}_2 (\hat{n} \cdot \vec{v}_1)^2 + \frac{32}{3} \hat{n} \times \vec{S}_1 \cdot \vec{v}_1 \hat{n} \cdot \vec{a}_2 (\hat{n} \cdot \vec{v}_1)^2 + \right. \\
 & 4 \hat{n} \times \vec{S}_1 \cdot \vec{v}_1 \hat{n} \cdot \vec{v}_2 (\hat{n} \cdot \vec{v}_1)^2 + 4 \hat{n} \times \vec{S}_1 \cdot \vec{a}_1 \hat{n} \cdot \vec{v}_2 (\hat{n} \cdot \vec{v}_1)^2 - \frac{64}{3} \hat{n} \times \vec{S}_1 \cdot \vec{v}_1 (\hat{n} \cdot \vec{v}_2)^2 \hat{n} \cdot \vec{v}_1 - \\
 & \frac{64}{3} \hat{n} \times \vec{S}_1 \cdot \vec{a}_1 (\hat{n} \cdot \vec{v}_2)^2 \hat{n} \cdot \vec{v}_1 - \frac{2}{3} \vec{S}_1 \times \vec{v}_1 \cdot \vec{v}_2 \hat{n} \cdot \vec{a}_1 \hat{n} \cdot \vec{v}_1 + \frac{32}{3} \vec{S}_1 \times \vec{v}_1 \cdot \vec{v}_2 \hat{n} \cdot \vec{v}_2 \hat{n} \cdot \vec{v}_1 + \frac{32}{3} \vec{S}_1 \times \vec{a}_1 \cdot \vec{v}_2 \hat{n} \cdot \vec{v}_2 \hat{n} \cdot \vec{v}_1 + \\
 & \left. \frac{10}{3} \vec{S}_1 \times \vec{v}_1 \cdot \vec{a}_1 \hat{n} \cdot \vec{v}_2 \hat{n} \cdot \vec{v}_1 + \frac{8}{3} \hat{n} \times \vec{S}_1 \cdot \vec{v}_1 \hat{n} \cdot \vec{a}_1 \hat{n} \cdot \vec{v}_2 \hat{n} \cdot \vec{v}_1 - \frac{2}{3} \hat{n} \times \vec{S}_1 \cdot \vec{v}_1 \vec{a}_1 \cdot \vec{v}_2 \hat{n} \cdot \vec{v}_1 - \frac{16}{3} \hat{n} \times \vec{S}_1 \cdot \vec{v}_1 \vec{v}_1 \cdot \vec{a}_2 \hat{n} \cdot \vec{v}_1 - \right.
 \end{aligned}$$

$$\begin{aligned}
& 2 \hat{n} \times \vec{S}_1 \cdot \vec{v}_1 \vec{v}_1 \cdot \vec{v}_2 \hat{n} \cdot \vec{v}_1 - 2 \hat{n} \times \vec{S}_1 \cdot \vec{a}_1 \vec{v}_1 \cdot \vec{v}_2 \hat{n} \cdot \vec{v}_1 + \frac{16}{3} \hat{n} \times \vec{S}_1 \cdot \vec{v}_1 \vec{v}_2 \cdot \vec{v}_2 \hat{n} \cdot \vec{v}_1 + \frac{16}{3} \hat{n} \times \vec{S}_1 \cdot \vec{a}_1 \vec{v}_2 \cdot \vec{v}_2 \hat{n} \cdot \vec{v}_1 - \\
& \frac{8}{3} \vec{S}_1 \times \vec{v}_1 \cdot \vec{a}_1 (\hat{n} \cdot \vec{v}_2)^2 - \frac{32}{3} \hat{n} \times \vec{S}_1 \cdot \vec{v}_1 \hat{n} \cdot \vec{a}_1 (\hat{n} \cdot \vec{v}_2)^2 + \frac{16}{3} \vec{S}_1 \times \vec{v}_1 \cdot \vec{v}_2 \hat{n} \cdot \vec{a}_1 \hat{n} \cdot \vec{v}_2 - \frac{8}{3} \vec{S}_1 \times \vec{v}_1 \cdot \vec{v}_2 \vec{a}_1 \cdot \vec{v}_2 + \\
& \frac{16}{3} \hat{n} \times \vec{S}_1 \cdot \vec{v}_1 \hat{n} \cdot \vec{v}_2 \vec{a}_1 \cdot \vec{v}_2 + \frac{4}{3} \vec{S}_1 \times \vec{v}_1 \cdot \vec{v}_2 \vec{v}_1 \cdot \vec{a}_1 - \frac{8}{3} \hat{n} \times \vec{S}_1 \cdot \vec{v}_1 \hat{n} \cdot \vec{v}_2 \vec{v}_1 \cdot \vec{a}_1 + \frac{1}{3} \vec{S}_1 \times \vec{v}_1 \cdot \vec{v}_2 \vec{v}_1 \cdot \vec{v}_1 + \vec{S}_1 \times \vec{a}_1 \cdot \vec{v}_2 \vec{v}_1 \cdot \vec{v}_1 + \\
& \frac{4}{3} \vec{S}_1 \times \vec{v}_1 \cdot \vec{a}_2 \vec{v}_1 \cdot \vec{v}_1 - \frac{8}{3} \hat{n} \times \vec{S}_1 \cdot \vec{v}_1 \hat{n} \cdot \vec{a}_2 \vec{v}_1 \cdot \vec{v}_1 - 2 \hat{n} \times \vec{S}_1 \cdot \vec{v}_1 \hat{n} \cdot \vec{v}_2 \vec{v}_1 \cdot \vec{v}_1 - 2 \hat{n} \times \vec{S}_1 \cdot \vec{a}_1 \hat{n} \cdot \vec{v}_2 \vec{v}_1 \cdot \vec{v}_1 - \\
& \frac{16}{3} \frac{1}{\vec{S}_1 \times \vec{v}_1 \cdot \vec{v}_2 \vec{v}_1 \cdot \vec{v}_2} - \frac{16}{3} \vec{S}_1 \times \vec{a}_1 \cdot \vec{v}_2 \vec{v}_1 \cdot \vec{v}_2 - \frac{5}{3} \vec{S}_1 \times \vec{v}_1 \cdot \vec{a}_1 \vec{v}_1 \cdot \vec{v}_2 - \frac{2}{3} \hat{n} \times \vec{S}_1 \cdot \vec{v}_1 \hat{n} \cdot \vec{a}_1 \vec{v}_1 \cdot \vec{v}_2 + \\
& \frac{32}{3} \hat{n} \times \vec{S}_1 \cdot \vec{v}_1 \hat{n} \cdot \vec{v}_2 \vec{v}_1 \cdot \vec{v}_2 + \frac{32}{3} \hat{n} \times \vec{S}_1 \cdot \vec{a}_1 \hat{n} \cdot \vec{v}_2 \vec{v}_1 \cdot \vec{v}_2 + \frac{4}{3} \vec{S}_1 \times \vec{v}_1 \cdot \vec{a}_1 \vec{v}_2 \cdot \vec{v}_2 + \frac{8}{3} \hat{n} \times \vec{S}_1 \cdot \vec{v}_1 \hat{n} \cdot \vec{a}_1 \vec{v}_2 \cdot \vec{v}_2 \Big) m_1 m_2 G^2 + \\
& \frac{1}{r^3} \left( \frac{4}{3} \vec{S}_1 \times \vec{v}_1 \cdot \vec{v}_2 (\hat{n} \cdot \vec{v}_1)^3 - 8 \hat{n} \times \vec{S}_1 \cdot \vec{v}_1 \hat{n} \cdot \vec{v}_2 (\hat{n} \cdot \vec{v}_1)^3 + 64 \hat{n} \times \vec{S}_1 \cdot \vec{v}_1 (\hat{n} \cdot \vec{v}_2)^2 (\hat{n} \cdot \vec{v}_1)^2 - \right. \\
& \frac{64}{3} \vec{S}_1 \times \vec{v}_1 \cdot \vec{v}_2 \hat{n} \cdot \vec{v}_2 (\hat{n} \cdot \vec{v}_1)^2 + 4 \hat{n} \times \vec{S}_1 \cdot \vec{v}_1 \vec{v}_1 \cdot \vec{v}_2 (\hat{n} \cdot \vec{v}_1)^2 - \frac{32}{3} \hat{n} \times \vec{S}_1 \cdot \vec{v}_1 \vec{v}_2 \cdot \vec{v}_2 (\hat{n} \cdot \vec{v}_1)^2 - \\
& 2 \vec{S}_1 \times \vec{v}_1 \cdot \vec{v}_2 \vec{v}_1 \cdot \vec{v}_1 \hat{n} \cdot \vec{v}_1 + 8 \hat{n} \times \vec{S}_1 \cdot \vec{v}_1 \hat{n} \cdot \vec{v}_2 \vec{v}_1 \cdot \vec{v}_1 \hat{n} \cdot \vec{v}_1 + \frac{32}{3} \vec{S}_1 \times \vec{v}_1 \cdot \vec{v}_2 \vec{v}_1 \cdot \vec{v}_2 \hat{n} \cdot \vec{v}_1 - \\
& \frac{128}{3} \hat{n} \times \vec{S}_1 \cdot \vec{v}_1 \hat{n} \cdot \vec{v}_2 \vec{v}_1 \cdot \vec{v}_2 \hat{n} \cdot \vec{v}_1 + \frac{16}{3} \hat{n} \times \vec{S}_1 \cdot \vec{v}_1 (\vec{v}_1 \cdot \vec{v}_2)^2 - \frac{32}{3} \hat{n} \times \vec{S}_1 \cdot \vec{v}_1 (\hat{n} \cdot \vec{v}_2)^2 \vec{v}_1 \cdot \vec{v}_1 + \\
& \left. \frac{16}{3} \vec{S}_1 \times \vec{v}_1 \cdot \vec{v}_2 \hat{n} \cdot \vec{v}_2 \vec{v}_1 \cdot \vec{v}_1 - 2 \hat{n} \times \vec{S}_1 \cdot \vec{v}_1 \vec{v}_1 \cdot \vec{v}_1 \vec{v}_1 \cdot \vec{v}_2 + \frac{8}{3} \hat{n} \times \vec{S}_1 \cdot \vec{v}_1 \vec{v}_1 \cdot \vec{v}_1 \vec{v}_2 \cdot \vec{v}_2 \right) m_1 m_2 G^2 + \\
& m_1 m_2 \left( \frac{8}{3} \log \left( \frac{r}{R_\theta} \right) \frac{1}{\vec{S}_1 \times \vec{a}_1 \cdot \vec{a}_2} - \frac{16}{9} \frac{1}{\vec{S}_1 \times \vec{a}_1 \cdot \vec{a}_2} - \frac{8}{9} \frac{2}{\vec{S}_1 \times \vec{v}_1 \cdot \vec{a}_2} - \frac{8}{9} \frac{1}{\vec{S}_1 \times \vec{a}_1 \cdot \vec{a}_2} + \frac{8}{3} \hat{n} \times \vec{S}_1 \cdot \vec{a}_1 \hat{n} \cdot \vec{a}_2 + \right. \\
& \frac{4}{3} \hat{n} \times \vec{S}_1 \cdot \vec{v}_1 \hat{n} \cdot \vec{a}_2 + \frac{4}{3} \hat{n} \times \vec{S}_1 \cdot \vec{a}_1 \hat{n} \cdot \vec{a}_2 + \frac{4}{3} \frac{2}{\vec{S}_1 \times \vec{v}_1 \cdot \vec{a}_2} \log \left( \frac{r}{R_\theta} \right) + \\
& \left. \frac{4}{3} \frac{1}{\vec{S}_1 \times \vec{a}_1 \cdot \vec{a}_2} \log \left( \frac{r}{R_\theta} \right) + \frac{-\frac{4}{3} \frac{1}{\vec{S}_1 \times \vec{a}_1 \cdot \vec{a}_2} - \frac{2}{3} \frac{2}{\vec{S}_1 \times \vec{v}_1 \cdot \vec{a}_2} - \frac{2}{3} \frac{1}{\vec{S}_1 \times \vec{a}_1 \cdot \vec{a}_2}}{\epsilon_d} \right) G^2 \Big\}
\end{aligned}$$

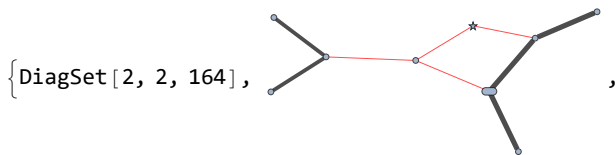

$$\begin{aligned}
& \frac{1}{r} \left( \hat{n} \times \vec{S}_1 \cdot \vec{v}_1 (\hat{n} \cdot \vec{a}_1)^2 + \frac{4}{3} \frac{1}{\vec{S}_1 \times \vec{v}_1 \cdot \vec{v}_2} \hat{n} \cdot \vec{a}_1 + \frac{4}{3} \vec{S}_1 \times \vec{a}_1 \cdot \vec{v}_2 \hat{n} \cdot \vec{a}_1 + 2 \vec{S}_1 \times \vec{v}_1 \cdot \vec{a}_1 \hat{n} \cdot \vec{a}_1 + \frac{2}{3} \vec{S}_1 \times \vec{v}_1 \cdot \vec{a}_2 \hat{n} \cdot \vec{a}_1 - \right. \\
& \frac{4}{3} \hat{n} \times \vec{S}_1 \cdot \vec{v}_1 \hat{n} \cdot \vec{a}_2 \hat{n} \cdot \vec{a}_1 + 2 \hat{n} \times \vec{S}_1 \cdot \vec{v}_1 \hat{n} \cdot \vec{v}_1 \hat{n} \cdot \vec{a}_1 + 2 \hat{n} \times \vec{S}_1 \cdot \vec{a}_1 \hat{n} \cdot \vec{v}_1 \hat{n} \cdot \vec{a}_1 - \frac{8}{3} \hat{n} \times \vec{S}_1 \cdot \vec{v}_1 \hat{n} \cdot \vec{v}_2 \hat{n} \cdot \vec{a}_1 - \\
& \frac{8}{3} \hat{n} \times \vec{S}_1 \cdot \vec{a}_1 \hat{n} \cdot \vec{v}_2 \hat{n} \cdot \vec{a}_1 + \frac{2}{3} \hat{n} \times \vec{S}_1 \cdot \vec{a}_1 (\hat{n} \cdot \vec{v}_1)^2 + \frac{1}{3} \hat{n} \times \vec{S}_1 \cdot \vec{v}_1 (\hat{n} \cdot \vec{v}_1)^2 + \frac{1}{3} \hat{n} \times \vec{S}_1 \cdot \vec{a}_1 (\hat{n} \cdot \vec{v}_1)^2 + \\
& \frac{4}{3} \frac{1}{\vec{S}_1 \times \vec{a}_1 \cdot \vec{v}_2} \hat{n} \cdot \vec{v}_1 + \frac{2}{3} \frac{1}{\vec{S}_1 \times \vec{v}_1 \cdot \vec{a}_1} \hat{n} \cdot \vec{v}_1 + \frac{2}{3} \frac{1}{\vec{S}_1 \times \vec{v}_1 \cdot \vec{a}_2} \hat{n} \cdot \vec{v}_1 + \frac{2}{3} \frac{2}{\vec{S}_1 \times \vec{v}_1 \cdot \vec{v}_2} \hat{n} \cdot \vec{v}_1 + \frac{2}{3} \frac{1}{\vec{S}_1 \times \vec{a}_1 \cdot \vec{v}_2} \hat{n} \cdot \vec{v}_1 + \\
& \frac{2}{3} \vec{S}_1 \times \vec{a}_1 \cdot \vec{a}_2 \hat{n} \cdot \vec{v}_1 - \frac{2}{3} \vec{S}_1 \times \vec{v}_1 \cdot \vec{a}_1 \hat{n} \cdot \vec{v}_1 - \frac{4}{3} \hat{n} \times \vec{S}_1 \cdot \vec{v}_1 \hat{n} \cdot \vec{a}_2 \hat{n} \cdot \vec{v}_1 - \frac{4}{3} \hat{n} \times \vec{S}_1 \cdot \vec{a}_1 \hat{n} \cdot \vec{a}_2 \hat{n} \cdot \vec{v}_1 + \\
& \frac{4}{3} \vec{S}_1 \times \vec{v}_1 \cdot \vec{a}_1 \hat{n} \cdot \vec{v}_2 - \frac{8}{3} \hat{n} \times \vec{S}_1 \cdot \vec{a}_1 \hat{n} \cdot \vec{v}_1 \hat{n} \cdot \vec{v}_2 - \frac{4}{3} \hat{n} \times \vec{S}_1 \cdot \vec{v}_1 \hat{n} \cdot \vec{v}_1 \hat{n} \cdot \vec{v}_2 - \frac{4}{3} \hat{n} \times \vec{S}_1 \cdot \vec{a}_1 \hat{n} \cdot \vec{v}_1 \hat{n} \cdot \vec{v}_2 + \\
& \left. \hat{n} \times \vec{S}_1 \cdot \vec{v}_1 \vec{a}_1 \cdot \vec{a}_1 + \frac{2}{3} \hat{n} \times \vec{S}_1 \cdot \vec{v}_1 \vec{a}_1 \cdot \vec{a}_2 + \frac{4}{3} \hat{n} \times \vec{S}_1 \cdot \vec{v}_1 \vec{a}_1 \cdot \vec{v}_2 + \frac{4}{3} \hat{n} \times \vec{S}_1 \cdot \vec{a}_1 \vec{a}_1 \cdot \vec{v}_2 + 2 \hat{n} \times \vec{S}_1 \cdot \vec{v}_1 \vec{v}_1 \cdot \vec{a}_1 + \right.
\end{aligned}$$

$$\begin{aligned}
& 2 \hat{n} \times \vec{S}_1 \cdot \vec{a}_1 \vec{v}_1 \cdot \vec{a}_1 + \frac{2}{3} \hat{n} \times \vec{S}_1 \cdot \vec{v}_1 \vec{v}_1 \cdot \vec{a}_2 + \frac{2}{3} \hat{n} \times \vec{S}_1 \cdot \vec{a}_1 \vec{v}_1 \cdot \vec{a}_2 - \frac{10}{3} \hat{n} \times \vec{S}_1 \cdot \vec{a}_1 \vec{v}_1 \cdot \vec{v}_1 - \frac{5}{3} \hat{n} \times \vec{S}_1 \cdot \vec{v}_1 \vec{v}_1 \cdot \vec{v}_1 - \\
& \frac{5}{3} \hat{n} \times \vec{S}_1 \cdot \vec{a}_1 \vec{v}_1 \cdot \vec{v}_1 + \frac{4}{3} \hat{n} \times \vec{S}_1 \cdot \vec{a}_1 \vec{v}_1 \cdot \vec{v}_2 + \frac{2}{3} \hat{n} \times \vec{S}_1 \cdot \vec{v}_1 \vec{v}_1 \cdot \vec{v}_2 + \frac{2}{3} \hat{n} \times \vec{S}_1 \cdot \vec{a}_1 \vec{v}_1 \cdot \vec{v}_2 \Big) m_1 m_2 G^2 + \frac{1}{r^2} \\
& \left( -\frac{4}{3} \hat{n} \times \vec{S}_1 \cdot \vec{v}_1 (\hat{n} \cdot \vec{v}_1)^3 - \frac{4}{3} \hat{n} \times \vec{S}_1 \cdot \vec{a}_1 (\hat{n} \cdot \vec{v}_1)^3 - \frac{8}{3} \vec{S}_1 \times \vec{v}_1 \cdot \vec{v}_2 (\hat{n} \cdot \vec{v}_1)^2 - \frac{8}{3} \vec{S}_1 \times \vec{a}_1 \cdot \vec{v}_2 (\hat{n} \cdot \vec{v}_1)^2 - \right. \\
& \vec{S}_1 \times \vec{v}_1 \cdot \vec{a}_1 (\hat{n} \cdot \vec{v}_1)^2 - \frac{4}{3} \vec{S}_1 \times \vec{v}_1 \cdot \vec{a}_2 (\hat{n} \cdot \vec{v}_1)^2 - 4 \hat{n} \times \vec{S}_1 \cdot \vec{v}_1 \hat{n} \cdot \vec{a}_1 (\hat{n} \cdot \vec{v}_1)^2 + \frac{16}{3} \hat{n} \times \vec{S}_1 \cdot \vec{v}_1 \hat{n} \cdot \vec{a}_2 (\hat{n} \cdot \vec{v}_1)^2 + \\
& \frac{32}{3} \hat{n} \times \vec{S}_1 \cdot \vec{v}_1 \hat{n} \cdot \vec{v}_2 (\hat{n} \cdot \vec{v}_1)^2 + \frac{32}{3} \hat{n} \times \vec{S}_1 \cdot \vec{a}_1 \hat{n} \cdot \vec{v}_2 (\hat{n} \cdot \vec{v}_1)^2 - \frac{16}{3} \hat{n} \times \vec{S}_1 \cdot \vec{v}_1 (\hat{n} \cdot \vec{v}_2)^2 \hat{n} \cdot \vec{v}_1 - \\
& \frac{16}{3} \hat{n} \times \vec{S}_1 \cdot \vec{a}_1 (\hat{n} \cdot \vec{v}_2)^2 \hat{n} \cdot \vec{v}_1 - 3 \vec{S}_1 \times \vec{v}_1 \cdot \vec{v}_2 \hat{n} \cdot \vec{a}_1 \hat{n} \cdot \vec{v}_1 + \frac{8}{3} \vec{S}_1 \times \vec{v}_1 \cdot \vec{v}_2 \hat{n} \cdot \vec{v}_2 \hat{n} \cdot \vec{v}_1 + \frac{8}{3} \vec{S}_1 \times \vec{a}_1 \cdot \vec{v}_2 \hat{n} \cdot \vec{v}_2 \hat{n} \cdot \vec{v}_1 - \\
& \frac{2}{3} \vec{S}_1 \times \vec{v}_1 \cdot \vec{a}_1 \hat{n} \cdot \vec{v}_2 \hat{n} \cdot \vec{v}_1 + 12 \hat{n} \times \vec{S}_1 \cdot \vec{v}_1 \hat{n} \cdot \vec{a}_1 \hat{n} \cdot \vec{v}_2 \hat{n} \cdot \vec{v}_1 - 3 \hat{n} \times \vec{S}_1 \cdot \vec{v}_1 \vec{a}_1 \cdot \vec{v}_2 \hat{n} \cdot \vec{v}_1 - 4 \hat{n} \times \vec{S}_1 \cdot \vec{v}_1 \vec{v}_1 \cdot \vec{a}_1 \hat{n} \cdot \vec{v}_1 - \\
& \frac{8}{3} \hat{n} \times \vec{S}_1 \cdot \vec{v}_1 \vec{v}_1 \cdot \vec{a}_2 \hat{n} \cdot \vec{v}_1 + 4 \hat{n} \times \vec{S}_1 \cdot \vec{v}_1 \vec{v}_1 \cdot \vec{v}_1 \hat{n} \cdot \vec{v}_1 + 4 \hat{n} \times \vec{S}_1 \cdot \vec{a}_1 \vec{v}_1 \cdot \vec{v}_1 \hat{n} \cdot \vec{v}_1 - \frac{16}{3} \hat{n} \times \vec{S}_1 \cdot \vec{v}_1 \vec{v}_1 \cdot \vec{v}_2 \hat{n} \cdot \vec{v}_1 - \\
& \frac{16}{3} \hat{n} \times \vec{S}_1 \cdot \vec{a}_1 \vec{v}_1 \cdot \vec{v}_2 \hat{n} \cdot \vec{v}_1 + \frac{4}{3} \hat{n} \times \vec{S}_1 \cdot \vec{v}_1 \vec{v}_2 \cdot \vec{v}_2 \hat{n} \cdot \vec{v}_1 + \frac{4}{3} \hat{n} \times \vec{S}_1 \cdot \vec{a}_1 \vec{v}_2 \cdot \vec{v}_2 \hat{n} \cdot \vec{v}_1 - \frac{16}{3} \hat{n} \times \vec{S}_1 \cdot \vec{v}_1 \hat{n} \cdot \vec{a}_1 (\hat{n} \cdot \vec{v}_2)^2 + \\
& \frac{8}{3} \vec{S}_1 \times \vec{v}_1 \cdot \vec{v}_2 \hat{n} \cdot \vec{a}_1 \hat{n} \cdot \vec{v}_2 - \frac{4}{3} \vec{S}_1 \times \vec{v}_1 \cdot \vec{v}_2 \vec{a}_1 \cdot \vec{v}_2 + \frac{8}{3} \hat{n} \times \vec{S}_1 \cdot \vec{v}_1 \hat{n} \cdot \vec{v}_2 \vec{a}_1 \cdot \vec{v}_2 - 3 \vec{S}_1 \times \vec{v}_1 \cdot \vec{v}_2 \vec{v}_1 \cdot \vec{a}_1 + \\
& 6 \hat{n} \times \vec{S}_1 \cdot \vec{v}_1 \hat{n} \cdot \vec{v}_2 \vec{v}_1 \cdot \vec{a}_1 + \frac{4}{3} \vec{S}_1 \times \vec{v}_1 \cdot \vec{v}_2 \vec{v}_1 \cdot \vec{v}_1 + \frac{4}{3} \vec{S}_1 \times \vec{a}_1 \cdot \vec{v}_2 \vec{v}_1 \cdot \vec{v}_1 - \vec{S}_1 \times \vec{v}_1 \cdot \vec{a}_1 \vec{v}_1 \cdot \vec{v}_1 + \frac{2}{3} \vec{S}_1 \times \vec{v}_1 \cdot \vec{a}_2 \vec{v}_1 \cdot \vec{v}_1 + \\
& 4 \hat{n} \times \vec{S}_1 \cdot \vec{v}_1 \hat{n} \cdot \vec{a}_1 \vec{v}_1 \cdot \vec{v}_1 - \frac{4}{3} \hat{n} \times \vec{S}_1 \cdot \vec{v}_1 \hat{n} \cdot \vec{a}_2 \vec{v}_1 \cdot \vec{v}_1 - \frac{8}{3} \hat{n} \times \vec{S}_1 \cdot \vec{v}_1 \hat{n} \cdot \vec{v}_2 \vec{v}_1 \cdot \vec{v}_1 - \frac{8}{3} \hat{n} \times \vec{S}_1 \cdot \vec{a}_1 \hat{n} \cdot \vec{v}_2 \vec{v}_1 \cdot \vec{v}_1 - \\
& \frac{4}{3} \vec{S}_1 \times \vec{v}_1 \cdot \vec{v}_2 \vec{v}_1 \cdot \vec{v}_2 - \frac{4}{3} \vec{S}_1 \times \vec{a}_1 \cdot \vec{v}_2 \vec{v}_1 \cdot \vec{v}_2 + \frac{1}{3} \vec{S}_1 \times \vec{v}_1 \cdot \vec{a}_1 \vec{v}_1 \cdot \vec{v}_2 - 3 \hat{n} \times \vec{S}_1 \cdot \vec{v}_1 \hat{n} \cdot \vec{a}_1 \vec{v}_1 \cdot \vec{v}_2 + \\
& \frac{8}{3} \hat{n} \times \vec{S}_1 \cdot \vec{v}_1 \hat{n} \cdot \vec{v}_2 \vec{v}_1 \cdot \vec{v}_2 + \frac{8}{3} \hat{n} \times \vec{S}_1 \cdot \vec{a}_1 \hat{n} \cdot \vec{v}_2 \vec{v}_1 \cdot \vec{v}_2 + \frac{4}{3} \hat{n} \times \vec{S}_1 \cdot \vec{v}_1 \hat{n} \cdot \vec{a}_1 \vec{v}_2 \cdot \vec{v}_2 \Big) m_1 m_2 G^2 + \frac{1}{r^3} \\
& \left( \frac{5}{2} \hat{n} \times \vec{S}_1 \cdot \vec{v}_1 (\hat{n} \cdot \vec{v}_1)^4 + \frac{14}{3} \vec{S}_1 \times \vec{v}_1 \cdot \vec{v}_2 (\hat{n} \cdot \vec{v}_1)^3 - 28 \hat{n} \times \vec{S}_1 \cdot \vec{v}_1 \hat{n} \cdot \vec{v}_2 (\hat{n} \cdot \vec{v}_1)^3 + 32 \hat{n} \times \vec{S}_1 \cdot \vec{v}_1 (\hat{n} \cdot \vec{v}_2)^2 (\hat{n} \cdot \vec{v}_1)^2 - \right. \\
& \frac{32}{3} \vec{S}_1 \times \vec{v}_1 \cdot \vec{v}_2 \hat{n} \cdot \vec{v}_2 (\hat{n} \cdot \vec{v}_1)^2 - 7 \hat{n} \times \vec{S}_1 \cdot \vec{v}_1 \vec{v}_1 \cdot \vec{v}_1 (\hat{n} \cdot \vec{v}_1)^2 + 14 \hat{n} \times \vec{S}_1 \cdot \vec{v}_1 \vec{v}_1 \cdot \vec{v}_2 (\hat{n} \cdot \vec{v}_1)^2 - \\
& \frac{16}{3} \hat{n} \times \vec{S}_1 \cdot \vec{v}_1 \vec{v}_2 \cdot \vec{v}_2 (\hat{n} \cdot \vec{v}_1)^2 - 2 \vec{S}_1 \times \vec{v}_1 \cdot \vec{v}_2 \vec{v}_1 \cdot \vec{v}_1 \hat{n} \cdot \vec{v}_1 + 8 \hat{n} \times \vec{S}_1 \cdot \vec{v}_1 \hat{n} \cdot \vec{v}_2 \vec{v}_1 \cdot \vec{v}_1 \hat{n} \cdot \vec{v}_1 + \\
& \frac{16}{3} \vec{S}_1 \times \vec{v}_1 \cdot \vec{v}_2 \vec{v}_1 \cdot \vec{v}_2 \hat{n} \cdot \vec{v}_1 - \frac{64}{3} \hat{n} \times \vec{S}_1 \cdot \vec{v}_1 \hat{n} \cdot \vec{v}_2 \vec{v}_1 \cdot \vec{v}_2 \hat{n} \cdot \vec{v}_1 + \frac{1}{2} \hat{n} \times \vec{S}_1 \cdot \vec{v}_1 (\vec{v}_1 \cdot \vec{v}_1)^2 + \frac{8}{3} \hat{n} \times \vec{S}_1 \cdot \vec{v}_1 (\vec{v}_1 \cdot \vec{v}_2)^2 - \\
& \frac{16}{3} \hat{n} \times \vec{S}_1 \cdot \vec{v}_1 (\hat{n} \cdot \vec{v}_2)^2 \vec{v}_1 \cdot \vec{v}_1 + \frac{8}{3} \vec{S}_1 \times \vec{v}_1 \cdot \vec{v}_2 \hat{n} \cdot \vec{v}_2 \vec{v}_1 \cdot \vec{v}_1 - 2 \hat{n} \times \vec{S}_1 \cdot \vec{v}_1 \vec{v}_1 \cdot \vec{v}_1 \vec{v}_1 \cdot \vec{v}_2 + \frac{4}{3} \hat{n} \times \vec{S}_1 \cdot \vec{v}_1 \vec{v}_1 \cdot \vec{v}_1 \vec{v}_2 \cdot \vec{v}_2 \Big) \\
& m_1 m_2 G^2 + m_1 m_2 \left( \frac{4}{3} \log \left( \frac{r}{R_\theta} \right) \vec{S}_1 \times \vec{v}_1 \cdot \vec{a}_1 - \frac{8}{9} \vec{S}_1 \times \vec{v}_1 \cdot \vec{a}_1 + \frac{8}{9} \vec{S}_1 \times \vec{a}_1 \cdot \vec{a}_1 - \frac{4}{3} \hat{n} \times \vec{S}_1 \cdot \vec{a}_1 \hat{n} \cdot \vec{a}_1 - \right. \\
& \left. \frac{2}{3} \hat{n} \times \vec{S}_1 \cdot \vec{v}_1 \hat{n} \cdot \vec{a}_1 - \frac{2}{3} \hat{n} \times \vec{S}_1 \cdot \vec{a}_1 \hat{n} \cdot \vec{a}_1 - \frac{4}{3} \vec{S}_1 \times \vec{a}_1 \cdot \vec{a}_1 \log \left( \frac{r}{R_\theta} \right) + \frac{\frac{2}{3} \vec{S}_1 \times \vec{a}_1 \cdot \vec{a}_1 - \frac{2}{3} \vec{S}_1 \times \vec{v}_1 \cdot \vec{a}_1}{\epsilon_d} \right) G^2 \Big\}
\end{aligned}$$

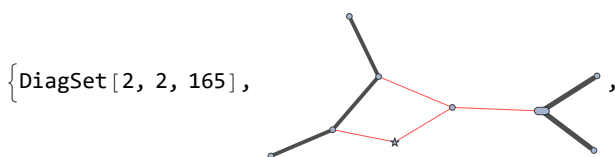



$$\frac{4}{3} \hat{n} \times \vec{S}_1 \cdot \vec{v}_1 \hat{n} \cdot \vec{a}_2 - \frac{8}{3} \hat{n} \times \vec{a}_1 \cdot \vec{S}_1 \hat{n} \cdot \vec{a}_2 + \frac{8}{3} \vec{a}_1 \times \vec{a}_2 \cdot \vec{S}_1 \log\left(\frac{r}{R_\theta}\right) +$$

$$\frac{4}{3} \vec{a}_2 \times \vec{S}_1 \cdot \vec{v}_1 \log\left(\frac{r}{R_\theta}\right) + \frac{-\frac{2}{3} \vec{a}_1 \times \vec{a}_2 \cdot \vec{S}_1 - \frac{4}{3} \vec{a}_1 \times \vec{a}_2 \cdot \vec{S}_1 - \frac{2}{3} \vec{a}_2 \times \vec{S}_1 \cdot \vec{v}_1}{\epsilon_d} m_2^2 \Bigg\}$$

{DiagSet[3, 1, 1], 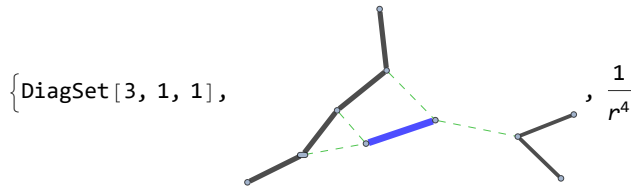,  $\frac{1}{r^4}$ }

$$G^3 m_1^2 m_2 \left( \frac{-\frac{48}{35} \hat{n} \cdot \vec{v}_1 \vec{S}_1 \times \vec{v}_1 \cdot \vec{v}_2 + \frac{48}{7} \hat{n} \cdot \vec{v}_2 \hat{n} \cdot \vec{v}_1 \hat{n} \times \vec{S}_1 \cdot \vec{v}_1 - \frac{48}{35} \vec{v}_1 \cdot \vec{v}_2 \hat{n} \times \vec{S}_1 \cdot \vec{v}_1}{\epsilon_d} + \right.$$

$$\frac{144}{35} \log\left(\frac{r}{R_\theta}\right) \hat{n} \cdot \vec{v}_1 \vec{S}_1 \times \vec{v}_1 \cdot \vec{v}_2 - \frac{144}{7} \log\left(\frac{r}{R_\theta}\right) \hat{n} \cdot \vec{v}_2 \hat{n} \cdot \vec{v}_1 \hat{n} \times \vec{S}_1 \cdot \vec{v}_1 + \frac{144}{35} \log\left(\frac{r}{R_\theta}\right) \vec{v}_1 \cdot \vec{v}_2 \hat{n} \times \vec{S}_1 \cdot \vec{v}_1 -$$

$$\left. \frac{6392 \hat{n} \cdot \vec{v}_1 \vec{S}_1 \times \vec{v}_1 \cdot \vec{v}_2}{1225} + \frac{1424}{49} \hat{n} \cdot \vec{v}_2 \hat{n} \cdot \vec{v}_1 \hat{n} \times \vec{S}_1 \cdot \vec{v}_1 - \frac{16}{5} \vec{v}_1 \cdot \vec{v}_1 \hat{n} \times \vec{S}_1 \cdot \vec{v}_2 + \frac{3408 \vec{v}_1 \cdot \vec{v}_2 \hat{n} \times \vec{S}_1 \cdot \vec{v}_1}{1225} \right\}$$

{DiagSet[3, 1, 2], 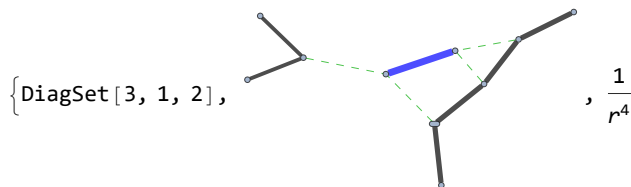,  $\frac{1}{r^4}$ }

$$G^3 m_1^2 m_2 \left( \frac{-24 (\hat{n} \cdot \vec{v}_1)^2 \hat{n} \times \vec{S}_1 \cdot \vec{v}_2 - \frac{48}{5} \hat{n} \cdot \vec{v}_1 \vec{S}_1 \times \vec{v}_1 \cdot \vec{v}_2 + \frac{24}{5} \vec{v}_1 \cdot \vec{v}_1 \hat{n} \times \vec{S}_1 \cdot \vec{v}_2}{\epsilon_d} + \right.$$

$$72 \log\left(\frac{r}{R_\theta}\right) (\hat{n} \cdot \vec{v}_1)^2 \hat{n} \times \vec{S}_1 \cdot \vec{v}_2 + \frac{144}{5} \log\left(\frac{r}{R_\theta}\right) \hat{n} \cdot \vec{v}_1 \vec{S}_1 \times \vec{v}_1 \cdot \vec{v}_2 - \frac{72}{5} \log\left(\frac{r}{R_\theta}\right) \vec{v}_1 \cdot \vec{v}_1 \hat{n} \times \vec{S}_1 \cdot \vec{v}_2 -$$

$$\left. 32 (\hat{n} \cdot \vec{v}_1)^2 \hat{n} \times \vec{S}_1 \cdot \vec{v}_2 - \frac{336}{25} \hat{n} \cdot \vec{v}_1 \vec{S}_1 \times \vec{v}_1 \cdot \vec{v}_2 + \frac{208}{25} \vec{v}_1 \cdot \vec{v}_1 \hat{n} \times \vec{S}_1 \cdot \vec{v}_2 - \frac{16}{5} \vec{v}_1 \cdot \vec{v}_2 \hat{n} \times \vec{S}_1 \cdot \vec{v}_1 \right\}$$

{DiagSet[3, 1, 3], 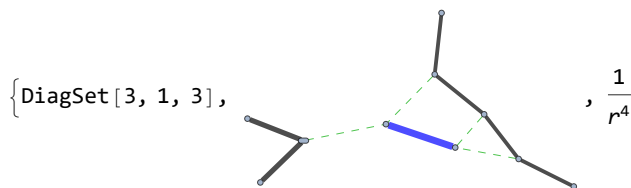,  $\frac{1}{r^4}$ }

$$G^3 m_2^3 \left( \frac{8 \vec{v}_2 \cdot \vec{v}_2 \hat{n} \times \vec{S}_1 \cdot \vec{v}_2 - 40 (\hat{n} \cdot \vec{v}_2)^2 \hat{n} \times \vec{S}_1 \cdot \vec{v}_2}{\epsilon_d} + 120 \log\left(\frac{r}{R_\theta}\right) (\hat{n} \cdot \vec{v}_2)^2 \hat{n} \times \vec{S}_1 \cdot \vec{v}_2 - \right.$$

$$\left. 24 \log\left(\frac{r}{R_\theta}\right) \vec{v}_2 \cdot \vec{v}_2 \hat{n} \times \vec{S}_1 \cdot \vec{v}_2 - 64 (\hat{n} \cdot \vec{v}_2)^2 \hat{n} \times \vec{S}_1 \cdot \vec{v}_2 + \frac{48}{5} \vec{v}_2 \cdot \vec{v}_2 \hat{n} \times \vec{S}_1 \cdot \vec{v}_2 \right\}$$

{DiagSet[3, 1, 4],

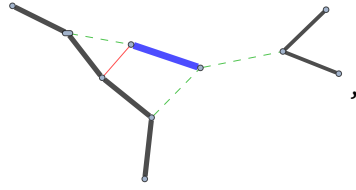

$$\frac{1}{r^3} G^3 m_1^2 m_2 \left( \frac{\frac{4}{5} \hat{n} \cdot \vec{v}_1 \hat{n} \times \vec{S}_1 \cdot \vec{v}_2 - 4 \hat{n} \cdot \vec{v}_2 \hat{n} \times \vec{S}_1 \cdot \vec{v}_1 + \frac{8}{5} \vec{S}_1 \times \vec{v}_1 \cdot \vec{v}_2}{\epsilon_d} - \right.$$

$$\frac{12}{5} \log\left(\frac{r}{R_\theta}\right) \hat{n} \cdot \vec{v}_1 \hat{n} \times \vec{S}_1 \cdot \vec{v}_2 + 12 \log\left(\frac{r}{R_\theta}\right) \hat{n} \cdot \vec{v}_2 \hat{n} \times \vec{S}_1 \cdot \vec{v}_1 + \frac{38}{25} \hat{n} \cdot \vec{v}_1 \hat{n} \times \vec{S}_1 \cdot \vec{v}_2 - 14 \hat{n} \cdot \vec{v}_2 \hat{n} \times \vec{S}_1 \cdot \vec{v}_1 -$$

$$\left. \frac{24}{5} \log\left(\frac{r}{R_\theta}\right) \vec{S}_1 \times \vec{v}_1 \cdot \vec{v}_2 + \frac{116}{25} \vec{S}_1 \times \vec{v}_1 \cdot \vec{v}_2 \right) + \frac{G^3 m_1^2 m_2 \left( -\frac{4}{5} \hat{n} \cdot \vec{v}_1 \vec{S}_1 \times \vec{v}_1 \cdot \vec{v}_2 - 4 \vec{v}_1 \cdot \vec{v}_2 \hat{n} \times \vec{S}_1 \cdot \vec{v}_1 \right)}{r^4} \Bigg\}$$

{DiagSet[3, 1, 5],

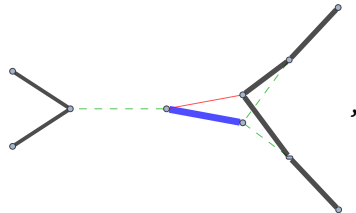

$$\frac{1}{r^3} m_1^2 m_2 \left( \frac{16}{5} \log\left(\frac{r}{R_\theta}\right) \vec{S}_1 \times \vec{v}_1 \cdot \vec{a}_2 - \frac{24}{25} \vec{S}_1 \times \vec{v}_1 \cdot \vec{a}_2 + \frac{194}{25} \hat{n} \times \vec{S}_1 \cdot \vec{v}_1 \hat{n} \cdot \vec{a}_2 - \frac{38}{25} \hat{n} \times \vec{S}_1 \cdot \vec{a}_2 \hat{n} \cdot \vec{v}_1 - \frac{36}{5} \hat{n} \times \vec{S}_1 \cdot \vec{v}_1 \hat{n} \cdot \vec{a}_2 \right.$$

$$\left. \log\left(\frac{r}{R_\theta}\right) + \frac{12}{5} \hat{n} \times \vec{S}_1 \cdot \vec{a}_2 \hat{n} \cdot \vec{v}_1 \log\left(\frac{r}{R_\theta}\right) + \frac{-\frac{16}{15} \vec{S}_1 \times \vec{v}_1 \cdot \vec{a}_2 + \frac{12}{5} \hat{n} \times \vec{S}_1 \cdot \vec{v}_1 \hat{n} \cdot \vec{a}_2 - \frac{4}{5} \hat{n} \times \vec{S}_1 \cdot \vec{a}_2 \hat{n} \cdot \vec{v}_1}{\epsilon_d} \right) G^3 + \frac{1}{r^4}$$

$$m_1^2 m_2 \left( 10 \hat{n} \times \vec{S}_1 \cdot \vec{v}_2 (\hat{n} \cdot \vec{v}_1)^2 - 12 \hat{n} \times \vec{S}_1 \cdot \vec{v}_2 \log\left(\frac{r}{R_\theta}\right) (\hat{n} \cdot \vec{v}_1)^2 + \frac{3354 \vec{S}_1 \times \vec{v}_1 \cdot \vec{v}_2 \hat{n} \cdot \vec{v}_1}{1225} - \frac{542}{49} \hat{n} \times \vec{S}_1 \cdot \vec{v}_1 \hat{n} \cdot \vec{v}_2 \hat{n} \cdot \vec{v}_1 - \right.$$

$$10 \hat{n} \times \vec{S}_1 \cdot \vec{v}_2 \hat{n} \cdot \vec{v}_2 \hat{n} \cdot \vec{v}_1 - \frac{228}{35} \vec{S}_1 \times \vec{v}_1 \cdot \vec{v}_2 \log\left(\frac{r}{R_\theta}\right) \hat{n} \cdot \vec{v}_1 + \frac{60}{7} \hat{n} \times \vec{S}_1 \cdot \vec{v}_1 \hat{n} \cdot \vec{v}_2 \log\left(\frac{r}{R_\theta}\right) \hat{n} \cdot \vec{v}_1 +$$

$$12 \hat{n} \times \vec{S}_1 \cdot \vec{v}_2 \hat{n} \cdot \vec{v}_2 \log\left(\frac{r}{R_\theta}\right) \hat{n} \cdot \vec{v}_1 + 46 \hat{n} \times \vec{S}_1 \cdot \vec{v}_1 (\hat{n} \cdot \vec{v}_2)^2 - \frac{346}{25} \vec{S}_1 \times \vec{v}_1 \cdot \vec{v}_2 \hat{n} \cdot \vec{v}_2 - \frac{38}{25} \hat{n} \times \vec{S}_1 \cdot \vec{v}_2 \vec{v}_1 \cdot \vec{v}_1 -$$

$$\frac{74}{245} \hat{n} \times \vec{S}_1 \cdot \vec{v}_1 \vec{v}_1 \cdot \vec{v}_2 + \frac{38}{25} \hat{n} \times \vec{S}_1 \cdot \vec{v}_2 \vec{v}_1 \cdot \vec{v}_2 - \frac{194}{25} \hat{n} \times \vec{S}_1 \cdot \vec{v}_1 \vec{v}_2 \cdot \vec{v}_2 - 36 \hat{n} \times \vec{S}_1 \cdot \vec{v}_1 (\hat{n} \cdot \vec{v}_2)^2 \log\left(\frac{r}{R_\theta}\right) +$$

$$\frac{84}{5} \vec{S}_1 \times \vec{v}_1 \cdot \vec{v}_2 \hat{n} \cdot \vec{v}_2 \log\left(\frac{r}{R_\theta}\right) + \frac{12}{5} \hat{n} \times \vec{S}_1 \cdot \vec{v}_2 \vec{v}_1 \cdot \vec{v}_1 \log\left(\frac{r}{R_\theta}\right) - \frac{12}{7} \hat{n} \times \vec{S}_1 \cdot \vec{v}_1 \vec{v}_1 \cdot \vec{v}_2 \log\left(\frac{r}{R_\theta}\right) -$$

$$\frac{12}{5} \hat{n} \times \vec{S}_1 \cdot \vec{v}_2 \vec{v}_1 \cdot \vec{v}_2 \log\left(\frac{r}{R_\theta}\right) + \frac{36}{5} \hat{n} \times \vec{S}_1 \cdot \vec{v}_1 \vec{v}_2 \cdot \vec{v}_2 \log\left(\frac{r}{R_\theta}\right) + \frac{1}{\epsilon_d} \left( 4 \hat{n} \times \vec{S}_1 \cdot \vec{v}_2 (\hat{n} \cdot \vec{v}_1)^2 + \frac{76}{35} \vec{S}_1 \times \vec{v}_1 \cdot \vec{v}_2 \hat{n} \cdot \vec{v}_1 - \right.$$

$$\frac{20}{7} \hat{n} \times \vec{S}_1 \cdot \vec{v}_1 \hat{n} \cdot \vec{v}_2 \hat{n} \cdot \vec{v}_1 - 4 \hat{n} \times \vec{S}_1 \cdot \vec{v}_2 \hat{n} \cdot \vec{v}_2 \hat{n} \cdot \vec{v}_1 + 12 \hat{n} \times \vec{S}_1 \cdot \vec{v}_1 (\hat{n} \cdot \vec{v}_2)^2 - \frac{28}{5} \vec{S}_1 \times \vec{v}_1 \cdot \vec{v}_2 \hat{n} \cdot \vec{v}_2 -$$

$$\left. \frac{4}{5} \hat{n} \times \vec{S}_1 \cdot \vec{v}_2 \vec{v}_1 \cdot \vec{v}_1 + \frac{4}{7} \hat{n} \times \vec{S}_1 \cdot \vec{v}_1 \vec{v}_1 \cdot \vec{v}_2 + \frac{4}{5} \hat{n} \times \vec{S}_1 \cdot \vec{v}_2 \vec{v}_1 \cdot \vec{v}_2 - \frac{12}{5} \hat{n} \times \vec{S}_1 \cdot \vec{v}_1 \vec{v}_2 \cdot \vec{v}_2 \right) G^3 \Bigg\}$$

{DiagSet[3, 1, 6],

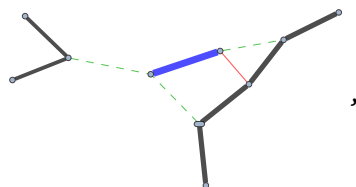

,  $\frac{1}{r^3}$



$$G^3 m_1^2 m_2 \left( \frac{-24 \hat{n} \cdot \vec{a}_1 \hat{n} \times \vec{S}_1 \cdot \vec{v}_2 - 8 \hat{n} \cdot \vec{v}_2 \hat{n} \times \vec{S}_1 \cdot \vec{a}_1 - \frac{16}{3} \vec{S}_1 \times \vec{a}_1 \cdot \vec{v}_2}{\epsilon_d} + 72 \log\left(\frac{r}{R_\theta}\right) \hat{n} \cdot \vec{a}_1 \hat{n} \times \vec{S}_1 \cdot \vec{v}_2 + \right. \\ \left. 24 \log\left(\frac{r}{R_\theta}\right) \hat{n} \cdot \vec{v}_2 \hat{n} \times \vec{S}_1 \cdot \vec{a}_1 - 56 \hat{n} \cdot \vec{a}_1 \hat{n} \times \vec{S}_1 \cdot \vec{v}_2 - 24 \hat{n} \cdot \vec{v}_2 \hat{n} \times \vec{S}_1 \cdot \vec{a}_1 + 16 \log\left(\frac{r}{R_\theta}\right) \vec{S}_1 \times \vec{a}_1 \cdot \vec{v}_2 - 16 \vec{S}_1 \times \vec{a}_1 \cdot \vec{v}_2 \right\}$$

{DiagSet[3, 1, 7],

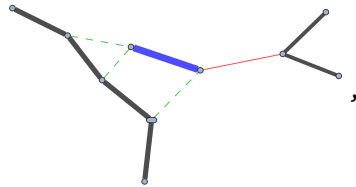

$$\frac{1}{r^4} G^3 m_1^2 m_2 \left( \frac{1}{\epsilon_d} \left( -24 (\hat{n} \cdot \vec{v}_1)^2 \hat{n} \times \vec{S}_1 \cdot \vec{v}_1 - \frac{24}{5} \hat{n} \cdot \vec{v}_1 \vec{S}_1 \times \vec{v}_1 \cdot \vec{v}_2 + 24 \hat{n} \cdot \vec{v}_2 \hat{n} \cdot \vec{v}_1 \hat{n} \times \vec{S}_1 \cdot \vec{v}_1 + \frac{24}{5} \vec{v}_1 \cdot \vec{v}_1 \hat{n} \times \vec{S}_1 \cdot \vec{v}_1 - \right. \right. \\ \left. \frac{24}{5} \vec{v}_1 \cdot \vec{v}_2 \hat{n} \times \vec{S}_1 \cdot \vec{v}_1 \right) + 72 \log\left(\frac{r}{R_\theta}\right) (\hat{n} \cdot \vec{v}_1)^2 \hat{n} \times \vec{S}_1 \cdot \vec{v}_1 + \frac{72}{5} \log\left(\frac{r}{R_\theta}\right) \hat{n} \cdot \vec{v}_1 \vec{S}_1 \times \vec{v}_1 \cdot \vec{v}_2 - 72 \log\left(\frac{r}{R_\theta}\right) \hat{n} \cdot \vec{v}_2 \\ \hat{n} \cdot \vec{v}_1 \hat{n} \times \vec{S}_1 \cdot \vec{v}_1 - \frac{72}{5} \log\left(\frac{r}{R_\theta}\right) \vec{v}_1 \cdot \vec{v}_1 \hat{n} \times \vec{S}_1 \cdot \vec{v}_1 + \frac{72}{5} \log\left(\frac{r}{R_\theta}\right) \vec{v}_1 \cdot \vec{v}_2 \hat{n} \times \vec{S}_1 \cdot \vec{v}_1 - 32 (\hat{n} \cdot \vec{v}_1)^2 \hat{n} \times \vec{S}_1 \cdot \vec{v}_1 - \\ \frac{88}{25} \hat{n} \cdot \vec{v}_1 \vec{S}_1 \times \vec{v}_1 \cdot \vec{v}_2 + 32 \hat{n} \cdot \vec{v}_2 \hat{n} \cdot \vec{v}_1 \hat{n} \times \vec{S}_1 \cdot \vec{v}_1 + \frac{148}{25} \vec{v}_1 \cdot \vec{v}_1 \hat{n} \times \vec{S}_1 \cdot \vec{v}_1 - \frac{88}{25} \vec{v}_1 \cdot \vec{v}_2 \hat{n} \times \vec{S}_1 \cdot \vec{v}_1 \Big) + \\ \left. \frac{G^3 m_1^2 m_2 \left( \frac{8 \hat{n} \cdot \vec{v}_1 \hat{n} \times \vec{S}_1 \cdot \vec{v}_1}{\epsilon_d} - 24 \log\left(\frac{r}{R_\theta}\right) \hat{n} \cdot \vec{v}_1 \hat{n} \times \vec{S}_1 \cdot \vec{v}_1 + 8 \hat{n} \cdot \vec{v}_1 \hat{n} \times \vec{S}_1 \cdot \vec{v}_1 \right)}{r^3} \right\}$$

{DiagSet[3, 1, 8],

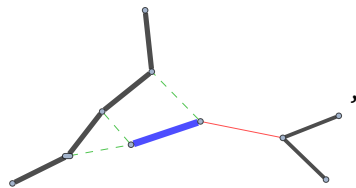

$$\frac{1}{r^3} G^3 m_1^2 m_2 \left( \frac{-\frac{12}{5} \hat{n} \cdot \vec{a}_1 \hat{n} \times \vec{S}_1 \cdot \vec{v}_1 + 4 \hat{n} \cdot \vec{v}_1 \hat{n} \times \vec{S}_1 \cdot \vec{a}_1 + \frac{32}{15} \vec{S}_1 \times \vec{v}_1 \cdot \vec{a}_1}{\epsilon_d} + \frac{36}{5} \log\left(\frac{r}{R_\theta}\right) \hat{n} \cdot \vec{a}_1 \hat{n} \times \vec{S}_1 \cdot \vec{v}_1 - \right. \\ \left. 12 \log\left(\frac{r}{R_\theta}\right) \hat{n} \cdot \vec{v}_1 \hat{n} \times \vec{S}_1 \cdot \vec{a}_1 - \frac{194}{25} \hat{n} \cdot \vec{a}_1 \hat{n} \times \vec{S}_1 \cdot \vec{v}_1 + 6 \hat{n} \cdot \vec{v}_1 \hat{n} \times \vec{S}_1 \cdot \vec{a}_1 - \frac{32}{5} \log\left(\frac{r}{R_\theta}\right) \vec{S}_1 \times \vec{v}_1 \cdot \vec{a}_1 + \frac{8}{25} \vec{S}_1 \times \vec{v}_1 \cdot \vec{a}_1 \right) + \\ \frac{1}{r^4} G^3 m_1^2 m_2 \left( \frac{1}{\epsilon_d} \left( -\frac{8}{7} (\hat{n} \cdot \vec{v}_1)^2 \hat{n} \times \vec{S}_1 \cdot \vec{v}_1 + \frac{8}{5} \hat{n} \cdot \vec{v}_1 \vec{S}_1 \times \vec{v}_1 \cdot \vec{v}_2 - 8 \hat{n} \cdot \vec{v}_2 \hat{n} \cdot \vec{v}_1 \hat{n} \times \vec{S}_1 \cdot \vec{v}_1 + \frac{8}{35} \vec{v}_1 \cdot \vec{v}_1 \hat{n} \times \vec{S}_1 \cdot \vec{v}_1 + \right. \right. \\ \left. \frac{8}{5} \vec{v}_1 \cdot \vec{v}_2 \hat{n} \times \vec{S}_1 \cdot \vec{v}_1 \right) + \frac{24}{7} \log\left(\frac{r}{R_\theta}\right) (\hat{n} \cdot \vec{v}_1)^2 \hat{n} \times \vec{S}_1 \cdot \vec{v}_1 - \frac{24}{5} \log\left(\frac{r}{R_\theta}\right) \hat{n} \cdot \vec{v}_1 \vec{S}_1 \times \vec{v}_1 \cdot \vec{v}_2 + 24 \log\left(\frac{r}{R_\theta}\right) \hat{n} \cdot \vec{v}_2 \\ \hat{n} \cdot \vec{v}_1 \hat{n} \times \vec{S}_1 \cdot \vec{v}_1 - \frac{24}{35} \log\left(\frac{r}{R_\theta}\right) \vec{v}_1 \cdot \vec{v}_1 \hat{n} \times \vec{S}_1 \cdot \vec{v}_1 - \frac{24}{5} \log\left(\frac{r}{R_\theta}\right) \vec{v}_1 \cdot \vec{v}_2 \hat{n} \times \vec{S}_1 \cdot \vec{v}_1 + \frac{52}{49} (\hat{n} \cdot \vec{v}_1)^2 \hat{n} \times \vec{S}_1 \cdot \vec{v}_1 + \\ \left. \frac{156}{25} \hat{n} \cdot \vec{v}_1 \vec{S}_1 \times \vec{v}_1 \cdot \vec{v}_2 - 36 \hat{n} \cdot \vec{v}_2 \hat{n} \cdot \vec{v}_1 \hat{n} \times \vec{S}_1 \cdot \vec{v}_1 + \frac{2232 \vec{v}_1 \cdot \vec{v}_1 \hat{n} \times \vec{S}_1 \cdot \vec{v}_1}{1225} + \frac{156}{25} \vec{v}_1 \cdot \vec{v}_2 \hat{n} \times \vec{S}_1 \cdot \vec{v}_1 \right) \Big\}$$

{DiagSet[3, 1, 9],

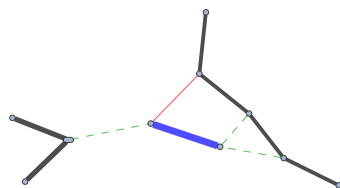

,  $\frac{1}{r^4} G^3 m_2^3$

$$\left( \frac{1}{\epsilon_d} \left( 40 (\hat{n} \cdot \vec{v}_2)^2 \hat{n} \times \vec{S}_1 \cdot \vec{v}_2 - 8 \hat{n} \cdot \vec{v}_2 \vec{S}_1 \times \vec{v}_1 \cdot \vec{v}_2 - 40 \hat{n} \cdot \vec{v}_1 \hat{n} \cdot \vec{v}_2 \hat{n} \times \vec{S}_1 \cdot \vec{v}_2 + 8 \vec{v}_1 \cdot \vec{v}_2 \hat{n} \times \vec{S}_1 \cdot \vec{v}_2 - 8 \vec{v}_2 \cdot \vec{v}_2 \hat{n} \times \vec{S}_1 \cdot \vec{v}_2 \right) - \right. \\ \left. 120 \log \left( \frac{r}{R_\theta} \right) (\hat{n} \cdot \vec{v}_2)^2 \hat{n} \times \vec{S}_1 \cdot \vec{v}_2 + 24 \log \left( \frac{r}{R_\theta} \right) \hat{n} \cdot \vec{v}_2 \vec{S}_1 \times \vec{v}_1 \cdot \vec{v}_2 + 120 \log \left( \frac{r}{R_\theta} \right) \hat{n} \cdot \vec{v}_1 \hat{n} \cdot \vec{v}_2 \hat{n} \times \vec{S}_1 \cdot \vec{v}_2 - \right. \\ \left. 24 \log \left( \frac{r}{R_\theta} \right) \vec{v}_1 \cdot \vec{v}_2 \hat{n} \times \vec{S}_1 \cdot \vec{v}_2 + 24 \log \left( \frac{r}{R_\theta} \right) \vec{v}_2 \cdot \vec{v}_2 \hat{n} \times \vec{S}_1 \cdot \vec{v}_2 + 64 (\hat{n} \cdot \vec{v}_2)^2 \hat{n} \times \vec{S}_1 \cdot \vec{v}_2 - \right. \\ \left. 8 \hat{n} \cdot \vec{v}_2 \vec{S}_1 \times \vec{v}_1 \cdot \vec{v}_2 - 64 \hat{n} \cdot \vec{v}_1 \hat{n} \cdot \vec{v}_2 \hat{n} \times \vec{S}_1 \cdot \vec{v}_2 + 8 \vec{v}_1 \cdot \vec{v}_2 \hat{n} \times \vec{S}_1 \cdot \vec{v}_2 - \frac{48}{5} \vec{v}_2 \cdot \vec{v}_2 \hat{n} \times \vec{S}_1 \cdot \vec{v}_2 \right) + \\ \left. \frac{G^3 m_2^3 \left( \frac{8 \hat{n} \cdot \vec{v}_2 \hat{n} \times \vec{S}_1 \cdot \vec{v}_2}{\epsilon_d} - 24 \log \left( \frac{r}{R_\theta} \right) \hat{n} \cdot \vec{v}_2 \hat{n} \times \vec{S}_1 \cdot \vec{v}_2 + 8 \hat{n} \cdot \vec{v}_2 \hat{n} \times \vec{S}_1 \cdot \vec{v}_2 \right)}{r^3} \right\}$$

$$\left\{ \text{DiagSet}[3, 1, 10], \right. \\ \left. \frac{1}{r^3} \right\}$$

$$G^3 m_2^3 \left( \frac{24 \hat{n} \cdot \vec{a}_2 \hat{n} \times \vec{S}_1 \cdot \vec{v}_2 + 8 \hat{n} \cdot \vec{v}_2 \hat{n} \times \vec{a}_2 \cdot \vec{S}_1 - \frac{32}{3} \vec{a}_2 \times \vec{S}_1 \cdot \vec{v}_2}{\epsilon_d} - 72 \log \left( \frac{r}{R_\theta} \right) \hat{n} \cdot \vec{a}_2 \hat{n} \times \vec{S}_1 \cdot \vec{v}_2 - \right. \\ \left. 24 \log \left( \frac{r}{R_\theta} \right) \hat{n} \cdot \vec{v}_2 \hat{n} \times \vec{a}_2 \cdot \vec{S}_1 + 72 \hat{n} \cdot \vec{a}_2 \hat{n} \times \vec{S}_1 \cdot \vec{v}_2 + 8 \hat{n} \cdot \vec{v}_2 \hat{n} \times \vec{a}_2 \cdot \vec{S}_1 + 32 \log \left( \frac{r}{R_\theta} \right) \vec{a}_2 \times \vec{S}_1 \cdot \vec{v}_2 - 16 \vec{a}_2 \times \vec{S}_1 \cdot \vec{v}_2 \right\}$$

$$\left\{ \text{DiagSet}[3, 1, 11], \right. \\ \left. \right\}$$

$$\frac{1}{r^3} G^3 m_1^2 m_2 \left( -\frac{4}{3} \vec{S}_1 \times \vec{v}_1 \cdot \vec{a}_2 + \frac{\frac{4}{5} \hat{n} \cdot \vec{v}_1 \hat{n} \times \vec{S}_1 \cdot \vec{v}_2 - \frac{4}{5} \hat{n} \cdot \vec{v}_2 \hat{n} \times \vec{S}_1 \cdot \vec{v}_1 - 4 \hat{n} \cdot \vec{v}_2 \hat{n} \times \vec{S}_1 \cdot \vec{v}_2 + \frac{8}{15} \vec{S}_1 \times \vec{v}_1 \cdot \vec{v}_2}{\epsilon_d} - \right. \\ \left. \frac{12}{5} \log \left( \frac{r}{R_\theta} \right) \hat{n} \cdot \vec{v}_1 \hat{n} \times \vec{S}_1 \cdot \vec{v}_2 + \frac{12}{5} \log \left( \frac{r}{R_\theta} \right) \hat{n} \cdot \vec{v}_2 \hat{n} \times \vec{S}_1 \cdot \vec{v}_1 + 12 \log \left( \frac{r}{R_\theta} \right) \hat{n} \cdot \vec{v}_2 \hat{n} \times \vec{S}_1 \cdot \vec{v}_2 + \right. \\ \left. \frac{98}{25} \hat{n} \cdot \vec{v}_1 \hat{n} \times \vec{S}_1 \cdot \vec{v}_2 - \frac{58}{25} \hat{n} \cdot \vec{v}_2 \hat{n} \times \vec{S}_1 \cdot \vec{v}_1 - 14 \hat{n} \cdot \vec{v}_2 \hat{n} \times \vec{S}_1 \cdot \vec{v}_2 - \frac{8}{5} \log \left( \frac{r}{R_\theta} \right) \vec{S}_1 \times \vec{v}_1 \cdot \vec{v}_2 + \frac{76}{75} \vec{S}_1 \times \vec{v}_1 \cdot \vec{v}_2 \right) + \\ \frac{G^3 m_1^2 m_2 \left( -\frac{4 \hat{n} \times \vec{S}_1 \cdot \vec{a}_2}{3 \epsilon_d} + 4 \log \left( \frac{r}{R_\theta} \right) \hat{n} \times \vec{S}_1 \cdot \vec{a}_2 - \frac{10}{3} \hat{n} \times \vec{S}_1 \cdot \vec{a}_2 \right)}{r^2} + \\ \frac{G^3 m_1^2 m_2 \left( \frac{12}{5} \hat{n} \cdot \vec{v}_1 \vec{S}_1 \times \vec{v}_1 \cdot \vec{v}_2 - 4 \hat{n} \cdot \vec{v}_2 \vec{S}_1 \times \vec{v}_1 \cdot \vec{v}_2 + \frac{4}{5} \vec{v}_1 \cdot \vec{v}_2 \hat{n} \times \vec{S}_1 \cdot \vec{v}_1 \right)}{r^4} \left\{ \right.$$

{DiagSet[3, 1, 12],

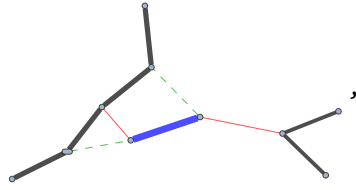

$$\frac{1}{r^3} G^3 m_1^2 m_2 \left( \frac{8}{3} \vec{S}_1 \times \vec{v}_1 \cdot \vec{a}_1 + \frac{4 \hat{n} \cdot \vec{v}_2 \hat{n} \times \vec{S}_1 \cdot \vec{v}_1 - \frac{4}{3} \vec{S}_1 \times \vec{v}_1 \cdot \vec{v}_2}{\epsilon_d} - 12 \log\left(\frac{r}{R_\theta}\right) \hat{n} \cdot \vec{v}_2 \hat{n} \times \vec{S}_1 \cdot \vec{v}_1 - \frac{8}{5} \hat{n} \cdot \vec{v}_1 \hat{n} \times \vec{S}_1 \cdot \vec{v}_1 + \right. \\ \left. 14 \hat{n} \cdot \vec{v}_2 \hat{n} \times \vec{S}_1 \cdot \vec{v}_1 + 4 \log\left(\frac{r}{R_\theta}\right) \vec{S}_1 \times \vec{v}_1 \cdot \vec{v}_2 - \frac{10}{3} \vec{S}_1 \times \vec{v}_1 \cdot \vec{v}_2 \right) + \frac{8 G^3 m_1^2 m_2 \hat{n} \times \vec{S}_1 \cdot \vec{a}_1}{3 r^2} - \frac{4 G^3 m_1^2 m_2 \vec{v}_1 \cdot \vec{v}_1 \hat{n} \times \vec{S}_1 \cdot \vec{v}_1}{5 r^4} \Bigg\}$$

{DiagSet[3, 1, 13],

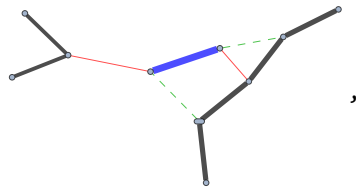

$$\frac{1}{r^3} G^3 m_1^2 m_2 \left( \frac{1}{\epsilon_d} \left( -\frac{24}{5} \hat{n} \cdot \vec{a}_1 \hat{n} \times \vec{S}_1 \cdot \vec{v}_1 - \frac{72}{5} \hat{n} \cdot \vec{v}_1 \hat{n} \times \vec{S}_1 \cdot \vec{a}_1 + 24 \hat{n} \cdot \vec{v}_2 \hat{n} \times \vec{S}_1 \cdot \vec{a}_1 - 8 \vec{S}_1 \times \vec{a}_1 \cdot \vec{v}_2 - \frac{16}{5} \vec{S}_1 \times \vec{v}_1 \cdot \vec{a}_1 \right) + \right. \\ \frac{72}{5} \log\left(\frac{r}{R_\theta}\right) \hat{n} \cdot \vec{a}_1 \hat{n} \times \vec{S}_1 \cdot \vec{v}_1 + \frac{216}{5} \log\left(\frac{r}{R_\theta}\right) \hat{n} \cdot \vec{v}_1 \hat{n} \times \vec{S}_1 \cdot \vec{a}_1 - 72 \log\left(\frac{r}{R_\theta}\right) \hat{n} \cdot \vec{v}_2 \hat{n} \times \vec{S}_1 \cdot \vec{a}_1 - \\ \frac{208}{25} \hat{n} \cdot \vec{a}_1 \hat{n} \times \vec{S}_1 \cdot \vec{v}_1 - \frac{864}{25} \hat{n} \cdot \vec{v}_1 \hat{n} \times \vec{S}_1 \cdot \vec{a}_1 + 56 \hat{n} \cdot \vec{v}_2 \hat{n} \times \vec{S}_1 \cdot \vec{a}_1 + \\ \left. 24 \log\left(\frac{r}{R_\theta}\right) \vec{S}_1 \times \vec{a}_1 \cdot \vec{v}_2 + \frac{48}{5} \log\left(\frac{r}{R_\theta}\right) \vec{S}_1 \times \vec{v}_1 \cdot \vec{a}_1 - \frac{32}{3} \vec{S}_1 \times \vec{a}_1 \cdot \vec{v}_2 - \frac{192}{25} \vec{S}_1 \times \vec{v}_1 \cdot \vec{a}_1 \right) + \\ \left. \frac{G^3 m_1^2 m_2 \left( \frac{16 \hat{n} \times \vec{S}_1 \cdot \vec{a}_1}{3 \epsilon_d} - 16 \log\left(\frac{r}{R_\theta}\right) \hat{n} \times \vec{S}_1 \cdot \vec{a}_1 + \frac{32}{3} \hat{n} \times \vec{S}_1 \cdot \vec{a}_1 \right)}{r^2} \right\}$$

{DiagSet[3, 1, 14],

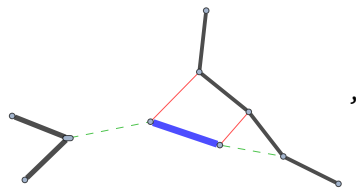

$$\frac{1}{r^3} G^3 m_2^3 \left( \frac{-8 \hat{n} \cdot \vec{a}_2 \hat{n} \times \vec{S}_1 \cdot \vec{v}_2 - 24 \hat{n} \cdot \vec{v}_1 \hat{n} \times \vec{a}_2 \cdot \vec{S}_1 + 8 \hat{n} \cdot \vec{v}_2 \hat{n} \times \vec{a}_2 \cdot \vec{S}_1 + 8 \vec{a}_2 \times \vec{S}_1 \cdot \vec{v}_1}{\epsilon_d} + \right. \\ 24 \log\left(\frac{r}{R_\theta}\right) \hat{n} \cdot \vec{a}_2 \hat{n} \times \vec{S}_1 \cdot \vec{v}_2 + 72 \log\left(\frac{r}{R_\theta}\right) \hat{n} \cdot \vec{v}_1 \hat{n} \times \vec{a}_2 \cdot \vec{S}_1 - 24 \log\left(\frac{r}{R_\theta}\right) \hat{n} \cdot \vec{v}_2 \hat{n} \times \vec{a}_2 \cdot \vec{S}_1 - 16 \hat{n} \cdot \vec{a}_2 \hat{n} \times \vec{S}_1 \cdot \vec{v}_2 - \\ 72 \hat{n} \cdot \vec{v}_1 \hat{n} \times \vec{a}_2 \cdot \vec{S}_1 + 32 \hat{n} \cdot \vec{v}_2 \hat{n} \times \vec{a}_2 \cdot \vec{S}_1 - 24 \log\left(\frac{r}{R_\theta}\right) \vec{a}_2 \times \vec{S}_1 \cdot \vec{v}_1 + 16 \vec{a}_2 \times \vec{S}_1 \cdot \vec{v}_1 - \frac{16}{3} \vec{a}_2 \times \vec{S}_1 \cdot \vec{v}_2 \Bigg) + \\ \left. \frac{G^3 m_2^3 \left( \frac{8 \hat{n} \times \vec{a}_2 \cdot \vec{S}_1}{\epsilon_d} - 24 \log\left(\frac{r}{R_\theta}\right) \hat{n} \times \vec{a}_2 \cdot \vec{S}_1 + 16 \hat{n} \times \vec{a}_2 \cdot \vec{S}_1 \right)}{r^2} \right\}$$

$\{\text{DiagSet}[3, 1, 15],$  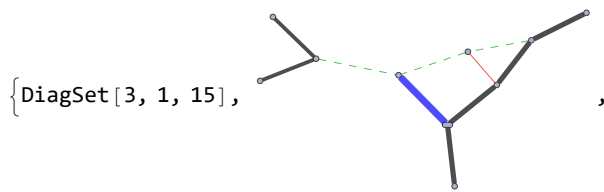 ,

$$\frac{G^3 m_1^2 m_2 \left( -\frac{16}{5} \hat{n} \cdot \vec{v}_1 \vec{S}_1 \times \vec{v}_1 \cdot \vec{v}_2 - \frac{64}{5} \vec{v}_1 \cdot \vec{v}_1 \hat{n} \times \vec{S}_1 \cdot \vec{v}_2 + 16 \vec{v}_1 \cdot \vec{v}_2 \hat{n} \times \vec{S}_1 \cdot \vec{v}_1 \right)}{r^4} \}$$

$\{\text{DiagSet}[3, 1, 16],$  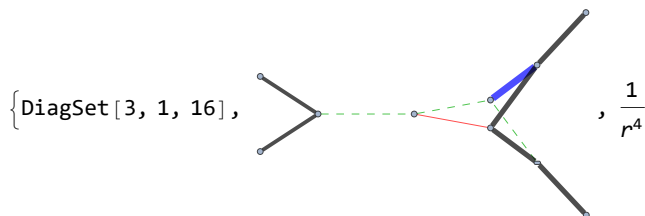 ,  $\frac{1}{r^4}$

$$G^3 m_1^2 m_2 \left( \frac{1}{\epsilon_d} \left( -\frac{192}{7} (\hat{n} \cdot \vec{v}_1)^2 \hat{n} \times \vec{S}_1 \cdot \vec{v}_2 - \frac{288}{35} \hat{n} \cdot \vec{v}_1 \vec{S}_1 \times \vec{v}_1 \cdot \vec{v}_2 - \frac{96}{7} \hat{n} \cdot \vec{v}_2 \hat{n} \cdot \vec{v}_1 \hat{n} \times \vec{S}_1 \cdot \vec{v}_1 + \right. \right. \\ \left. \frac{192}{35} \vec{v}_1 \cdot \vec{v}_1 \hat{n} \times \vec{S}_1 \cdot \vec{v}_2 + \frac{96}{35} \vec{v}_1 \cdot \vec{v}_2 \hat{n} \times \vec{S}_1 \cdot \vec{v}_1 \right) + \frac{576}{7} \log\left(\frac{r}{R_0}\right) (\hat{n} \cdot \vec{v}_1)^2 \hat{n} \times \vec{S}_1 \cdot \vec{v}_2 + \\ \frac{864}{35} \log\left(\frac{r}{R_0}\right) \hat{n} \cdot \vec{v}_1 \vec{S}_1 \times \vec{v}_1 \cdot \vec{v}_2 + \frac{288}{7} \log\left(\frac{r}{R_0}\right) \hat{n} \cdot \vec{v}_2 \hat{n} \cdot \vec{v}_1 \hat{n} \times \vec{S}_1 \cdot \vec{v}_1 - \frac{576}{35} \log\left(\frac{r}{R_0}\right) \vec{v}_1 \cdot \vec{v}_1 \hat{n} \times \vec{S}_1 \cdot \vec{v}_2 - \\ \frac{288}{35} \log\left(\frac{r}{R_0}\right) \vec{v}_1 \cdot \vec{v}_2 \hat{n} \times \vec{S}_1 \cdot \vec{v}_1 + \frac{128}{49} (\hat{n} \cdot \vec{v}_1)^2 \hat{n} \times \vec{S}_1 \cdot \vec{v}_2 + \frac{6588 \hat{n} \cdot \vec{v}_1 \vec{S}_1 \times \vec{v}_1 \cdot \vec{v}_2}{1225} - \\ \left. \frac{1952}{49} \hat{n} \cdot \vec{v}_2 \hat{n} \cdot \vec{v}_1 \hat{n} \times \vec{S}_1 \cdot \vec{v}_1 + \frac{368 \vec{v}_1 \cdot \vec{v}_1 \hat{n} \times \vec{S}_1 \cdot \vec{v}_2}{1225} + \frac{1444 \vec{v}_1 \cdot \vec{v}_2 \hat{n} \times \vec{S}_1 \cdot \vec{v}_1}{1225} \right) \}$$

$\{\text{DiagSet}[3, 1, 17],$  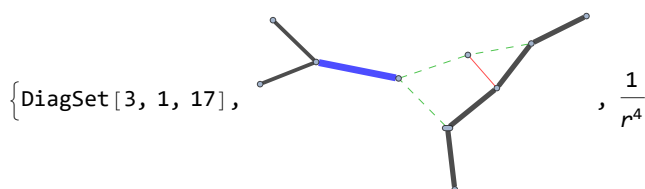 ,  $\frac{1}{r^4}$

$$G^3 m_1^2 m_2 \left( \frac{\left( \frac{48}{7} (\hat{n} \cdot \vec{v}_2)^2 \hat{n} \times \vec{S}_1 \cdot \vec{v}_1 - \frac{96}{35} \hat{n} \cdot \vec{v}_2 \vec{S}_1 \times \vec{v}_1 \cdot \vec{v}_2 - \frac{48}{35} \vec{v}_2 \cdot \vec{v}_2 \hat{n} \times \vec{S}_1 \cdot \vec{v}_1 \right)}{\epsilon_d} - \right. \\ \left. \frac{144}{7} \log\left(\frac{r}{R_0}\right) (\hat{n} \cdot \vec{v}_2)^2 \hat{n} \times \vec{S}_1 \cdot \vec{v}_1 + \frac{288}{35} \log\left(\frac{r}{R_0}\right) \hat{n} \cdot \vec{v}_2 \vec{S}_1 \times \vec{v}_1 \cdot \vec{v}_2 + \frac{144}{35} \log\left(\frac{r}{R_0}\right) \vec{v}_2 \cdot \vec{v}_2 \hat{n} \times \vec{S}_1 \cdot \vec{v}_1 + \right. \\ \left. \frac{640}{49} (\hat{n} \cdot \vec{v}_2)^2 \hat{n} \times \vec{S}_1 \cdot \vec{v}_1 - \frac{8864 \hat{n} \cdot \vec{v}_2 \vec{S}_1 \times \vec{v}_1 \cdot \vec{v}_2}{1225} + \frac{16}{5} \vec{v}_1 \cdot \vec{v}_2 \hat{n} \times \vec{S}_1 \cdot \vec{v}_2 - \frac{4432 \vec{v}_2 \cdot \vec{v}_2 \hat{n} \times \vec{S}_1 \cdot \vec{v}_1}{1225} \right) \}$$

$\{\text{DiagSet}[3, 1, 18],$  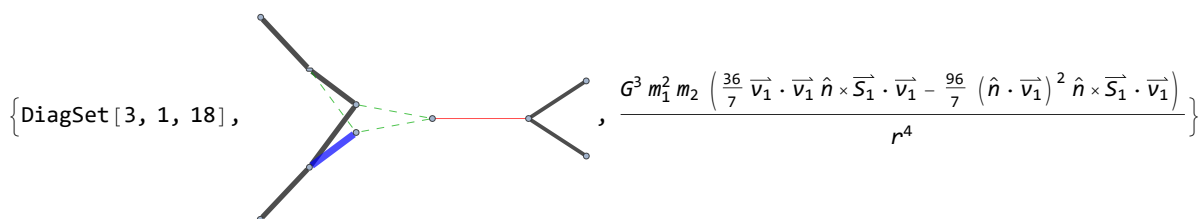 ,  $\frac{G^3 m_1^2 m_2 \left( \frac{36}{7} \vec{v}_1 \cdot \vec{v}_1 \hat{n} \times \vec{S}_1 \cdot \vec{v}_1 - \frac{96}{7} (\hat{n} \cdot \vec{v}_1)^2 \hat{n} \times \vec{S}_1 \cdot \vec{v}_1 \right)}{r^4} \}$

{DiagSet[3, 1, 19],

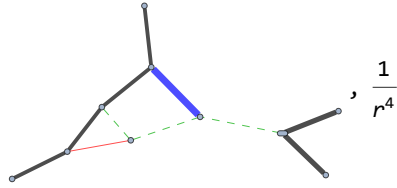

,  $\frac{1}{r^4}$

$$G^3 m_2^3 \left( \frac{16 \vec{v}_2 \cdot \vec{v}_2 \hat{n} \times \vec{S}_1 \cdot \vec{v}_2 - 80 (\hat{n} \cdot \vec{v}_2)^2 \hat{n} \times \vec{S}_1 \cdot \vec{v}_2}{\epsilon_d} + 240 \log\left(\frac{r}{R_\theta}\right) (\hat{n} \cdot \vec{v}_2)^2 \hat{n} \times \vec{S}_1 \cdot \vec{v}_2 - \right. \\ \left. 48 \log\left(\frac{r}{R_\theta}\right) \vec{v}_2 \cdot \vec{v}_2 \hat{n} \times \vec{S}_1 \cdot \vec{v}_2 - 128 (\hat{n} \cdot \vec{v}_2)^2 \hat{n} \times \vec{S}_1 \cdot \vec{v}_2 + 16 \vec{v}_2 \cdot \vec{v}_2 \hat{n} \times \vec{S}_1 \cdot \vec{v}_2 \right\}$$

{DiagSet[3, 1, 20],

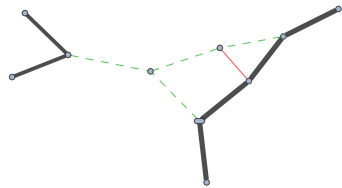

,

$$\frac{1}{r^3} m_1^2 m_2 \left( \frac{56}{5} \log\left(\frac{r}{R_\theta}\right) \vec{S}_1 \times \vec{v}_1 \cdot \vec{v}_2 + \frac{16}{25} \vec{S}_1 \times \vec{v}_1 \cdot \vec{v}_2 - \frac{16}{25} \vec{S}_1 \times \vec{a}_1 \cdot \vec{v}_2 + \frac{16}{25} \vec{S}_1 \times \vec{v}_1 \cdot \vec{a}_2 - 8 \hat{n} \times \vec{S}_1 \cdot \vec{v}_2 \hat{n} \cdot \vec{v}_1 + \right. \\ \frac{88}{25} \hat{n} \times \vec{S}_1 \cdot \vec{a}_2 \hat{n} \cdot \vec{v}_1 + \frac{112}{25} \hat{n} \times \vec{S}_1 \cdot \vec{v}_1 \hat{n} \cdot \vec{v}_2 + \frac{88}{25} \hat{n} \times \vec{S}_1 \cdot \vec{a}_1 \hat{n} \cdot \vec{v}_2 + \frac{24}{5} \vec{S}_1 \times \vec{a}_1 \cdot \vec{v}_2 \log\left(\frac{r}{R_\theta}\right) - \\ \frac{24}{5} \vec{S}_1 \times \vec{v}_1 \cdot \vec{a}_2 \log\left(\frac{r}{R_\theta}\right) + 24 \hat{n} \times \vec{S}_1 \cdot \vec{v}_2 \hat{n} \cdot \vec{v}_1 \log\left(\frac{r}{R_\theta}\right) - \frac{72}{5} \hat{n} \times \vec{S}_1 \cdot \vec{a}_2 \hat{n} \cdot \vec{v}_1 \log\left(\frac{r}{R_\theta}\right) - \\ \frac{48}{5} \hat{n} \times \vec{S}_1 \cdot \vec{v}_1 \hat{n} \cdot \vec{v}_2 \log\left(\frac{r}{R_\theta}\right) - \frac{72}{5} \hat{n} \times \vec{S}_1 \cdot \vec{a}_1 \hat{n} \cdot \vec{v}_2 \log\left(\frac{r}{R_\theta}\right) + \frac{1}{\epsilon_d} \left( -\frac{56}{15} \vec{S}_1 \times \vec{v}_1 \cdot \vec{v}_2 - \frac{8}{5} \vec{S}_1 \times \vec{a}_1 \cdot \vec{v}_2 + \right. \\ \left. \frac{8}{5} \vec{S}_1 \times \vec{v}_1 \cdot \vec{a}_2 - 8 \hat{n} \times \vec{S}_1 \cdot \vec{v}_2 \hat{n} \cdot \vec{v}_1 + \frac{24}{5} \hat{n} \times \vec{S}_1 \cdot \vec{a}_2 \hat{n} \cdot \vec{v}_1 + \frac{16}{5} \hat{n} \times \vec{S}_1 \cdot \vec{v}_1 \hat{n} \cdot \vec{v}_2 + \frac{24}{5} \hat{n} \times \vec{S}_1 \cdot \vec{a}_1 \hat{n} \cdot \vec{v}_2 \right) \Big) G^3 + \\ \frac{1}{r^4} m_1^2 m_2 \left( 32 \hat{n} \times \vec{S}_1 \cdot \vec{v}_2 (\hat{n} \cdot \vec{v}_1)^2 - 72 \hat{n} \times \vec{S}_1 \cdot \vec{v}_2 \log\left(\frac{r}{R_\theta}\right) (\hat{n} \cdot \vec{v}_1)^2 + \frac{17488 \vec{S}_1 \times \vec{v}_1 \cdot \vec{v}_2 \hat{n} \cdot \vec{v}_1}{1225} - \right. \\ \frac{1280}{49} \hat{n} \times \vec{S}_1 \cdot \vec{v}_1 \hat{n} \cdot \vec{v}_2 \hat{n} \cdot \vec{v}_1 + 32 \hat{n} \times \vec{S}_1 \cdot \vec{v}_2 \hat{n} \cdot \vec{v}_2 \hat{n} \cdot \vec{v}_1 - \frac{1296}{35} \vec{S}_1 \times \vec{v}_1 \cdot \vec{v}_2 \log\left(\frac{r}{R_\theta}\right) \hat{n} \cdot \vec{v}_1 + \\ \frac{288}{7} \hat{n} \times \vec{S}_1 \cdot \vec{v}_1 \hat{n} \cdot \vec{v}_2 \log\left(\frac{r}{R_\theta}\right) \hat{n} \cdot \vec{v}_1 - 72 \hat{n} \times \vec{S}_1 \cdot \vec{v}_2 \hat{n} \cdot \vec{v}_2 \log\left(\frac{r}{R_\theta}\right) \hat{n} \cdot \vec{v}_1 + \frac{168}{25} \vec{S}_1 \times \vec{v}_1 \cdot \vec{v}_2 \hat{n} \cdot \vec{v}_2 - \\ \frac{88}{25} \hat{n} \times \vec{S}_1 \cdot \vec{v}_2 \vec{v}_1 \cdot \vec{v}_1 - \frac{2896 \hat{n} \times \vec{S}_1 \cdot \vec{v}_1 \vec{v}_1 \cdot \vec{v}_2}{1225} - \frac{88}{25} \hat{n} \times \vec{S}_1 \cdot \vec{v}_2 \vec{v}_1 \cdot \vec{v}_2 - \frac{72}{5} \vec{S}_1 \times \vec{v}_1 \cdot \vec{v}_2 \hat{n} \cdot \vec{v}_2 \log\left(\frac{r}{R_\theta}\right) + \\ \frac{72}{5} \hat{n} \times \vec{S}_1 \cdot \vec{v}_2 \vec{v}_1 \cdot \vec{v}_1 \log\left(\frac{r}{R_\theta}\right) - \frac{288}{35} \hat{n} \times \vec{S}_1 \cdot \vec{v}_1 \vec{v}_1 \cdot \vec{v}_2 \log\left(\frac{r}{R_\theta}\right) + \frac{72}{5} \hat{n} \times \vec{S}_1 \cdot \vec{v}_2 \vec{v}_1 \cdot \vec{v}_2 \log\left(\frac{r}{R_\theta}\right) + \frac{1}{\epsilon_d} \\ \left( 24 \hat{n} \times \vec{S}_1 \cdot \vec{v}_2 (\hat{n} \cdot \vec{v}_1)^2 + \frac{432}{35} \vec{S}_1 \times \vec{v}_1 \cdot \vec{v}_2 \hat{n} \cdot \vec{v}_1 - \frac{96}{7} \hat{n} \times \vec{S}_1 \cdot \vec{v}_1 \hat{n} \cdot \vec{v}_2 \hat{n} \cdot \vec{v}_1 + 24 \hat{n} \times \vec{S}_1 \cdot \vec{v}_2 \hat{n} \cdot \vec{v}_2 \hat{n} \cdot \vec{v}_1 + \right. \\ \left. \frac{24}{5} \vec{S}_1 \times \vec{v}_1 \cdot \vec{v}_2 \hat{n} \cdot \vec{v}_2 - \frac{24}{5} \hat{n} \times \vec{S}_1 \cdot \vec{v}_2 \vec{v}_1 \cdot \vec{v}_1 + \frac{96}{35} \hat{n} \times \vec{S}_1 \cdot \vec{v}_1 \vec{v}_1 \cdot \vec{v}_2 - \frac{24}{5} \hat{n} \times \vec{S}_1 \cdot \vec{v}_2 \vec{v}_1 \cdot \vec{v}_2 \right) \Big) G^3 \Big\}$$

{DiagSet[3, 1, 21],

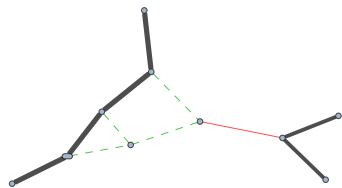

,

$$\begin{aligned}
& \frac{1}{r^3} G^3 m_1^2 m_2 \left( \frac{-\frac{12}{5} \hat{n} \cdot \vec{a}_1 \hat{n} \times \vec{S}_1 \cdot \vec{v}_1 + \frac{4}{5} \vec{S}_1 \times \vec{v}_1 \cdot \vec{a}_1 - \frac{4}{5} \hat{n} \cdot \vec{v}_1 \hat{n} \times \vec{S}_1 \cdot \vec{v}_1}{\epsilon_d} + \right. \\
& \frac{36}{5} \log\left(\frac{r}{R_\theta}\right) \hat{n} \cdot \vec{a}_1 \hat{n} \times \vec{S}_1 \cdot \vec{v}_1 - \frac{134}{25} \hat{n} \cdot \vec{a}_1 \hat{n} \times \vec{S}_1 \cdot \vec{v}_1 + \frac{36}{5} \hat{n} \cdot \vec{v}_1 \hat{n} \times \vec{S}_1 \cdot \vec{a}_1 - \\
& \left. \frac{12}{5} \log\left(\frac{r}{R_\theta}\right) \vec{S}_1 \times \vec{v}_1 \cdot \vec{a}_1 + \frac{98}{25} \vec{S}_1 \times \vec{v}_1 \cdot \vec{a}_1 + \frac{12}{5} \log\left(\frac{r}{R_\theta}\right) \hat{n} \cdot \vec{v}_1 \hat{n} \times \vec{S}_1 \cdot \vec{v}_1 - \frac{198}{25} \hat{n} \cdot \vec{v}_1 \hat{n} \times \vec{S}_1 \cdot \vec{v}_1 \right) + \\
& \frac{1}{r^4} G^3 m_1^2 m_2 \left( \frac{\frac{16}{7} (\hat{n} \cdot \vec{v}_1)^2 \hat{n} \times \vec{S}_1 \cdot \vec{v}_1 - \frac{16}{35} \vec{v}_1 \cdot \vec{v}_1 \hat{n} \times \vec{S}_1 \cdot \vec{v}_1}{\epsilon_d} - \frac{48}{7} \log\left(\frac{r}{R_\theta}\right) (\hat{n} \cdot \vec{v}_1)^2 \hat{n} \times \vec{S}_1 \cdot \vec{v}_1 + \right. \\
& \frac{48}{35} \log\left(\frac{r}{R_\theta}\right) \vec{v}_1 \cdot \vec{v}_1 \hat{n} \times \vec{S}_1 \cdot \vec{v}_1 + \frac{456}{49} (\hat{n} \cdot \vec{v}_1)^2 \hat{n} \times \vec{S}_1 \cdot \vec{v}_1 - \frac{24}{5} \hat{n} \cdot \vec{v}_1 \vec{S}_1 \times \vec{v}_1 \cdot \vec{v}_2 + \\
& \left. 24 \hat{n} \cdot \vec{v}_2 \hat{n} \cdot \vec{v}_1 \hat{n} \times \vec{S}_1 \cdot \vec{v}_1 + \frac{2536 \vec{v}_1 \cdot \vec{v}_1 \hat{n} \times \vec{S}_1 \cdot \vec{v}_1}{1225} - \frac{24}{5} \vec{v}_1 \cdot \vec{v}_2 \hat{n} \times \vec{S}_1 \cdot \vec{v}_1 \right) \Big\}
\end{aligned}$$

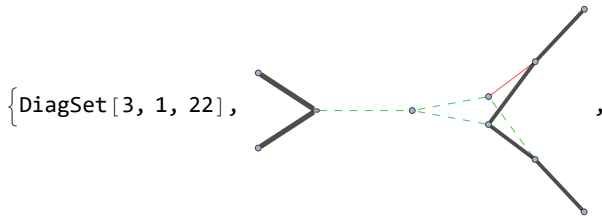

$$\begin{aligned}
& \frac{1}{r^3} G^3 m_2^3 \left( \frac{-48 \hat{n} \cdot \vec{v}_2 \hat{n} \times \vec{a}_2 \cdot \vec{S}_1 + 16 \vec{a}_2 \times \vec{S}_1 \cdot \vec{v}_2 - 24 \hat{n} \cdot \vec{v}_2 \hat{n} \times \vec{S}_1 \cdot \vec{v}_2}{\epsilon_d} + 144 \log\left(\frac{r}{R_\theta}\right) \hat{n} \cdot \vec{v}_2 \hat{n} \times \vec{a}_2 \cdot \vec{S}_1 - \right. \\
& 48 \hat{n} \cdot \vec{v}_2 \hat{n} \times \vec{a}_2 \cdot \vec{S}_1 - 48 \log\left(\frac{r}{R_\theta}\right) \vec{a}_2 \times \vec{S}_1 \cdot \vec{v}_2 + 72 \log\left(\frac{r}{R_\theta}\right) \hat{n} \cdot \vec{v}_2 \hat{n} \times \vec{S}_1 \cdot \vec{v}_2 - 24 \hat{n} \cdot \vec{v}_2 \hat{n} \times \vec{S}_1 \cdot \vec{v}_2 \Big) + \frac{1}{r^4} \\
& G^3 m_2^3 \left( \frac{1}{\epsilon_d} \left( 120 (\hat{n} \cdot \vec{v}_2)^2 \hat{n} \times \vec{S}_1 \cdot \vec{v}_2 + 24 \hat{n} \cdot \vec{v}_2 \vec{S}_1 \times \vec{v}_1 \cdot \vec{v}_2 + 120 \hat{n} \cdot \vec{v}_1 \hat{n} \cdot \vec{v}_2 \hat{n} \times \vec{S}_1 \cdot \vec{v}_2 - 24 \vec{v}_1 \cdot \vec{v}_2 \hat{n} \times \vec{S}_1 \cdot \vec{v}_2 - \right. \right. \\
& 24 \vec{v}_2 \cdot \vec{v}_2 \hat{n} \times \vec{S}_1 \cdot \vec{v}_2 \Big) - 360 \log\left(\frac{r}{R_\theta}\right) (\hat{n} \cdot \vec{v}_2)^2 \hat{n} \times \vec{S}_1 \cdot \vec{v}_2 - 72 \log\left(\frac{r}{R_\theta}\right) \hat{n} \cdot \vec{v}_2 \vec{S}_1 \times \vec{v}_1 \cdot \vec{v}_2 - 360 \log\left(\frac{r}{R_\theta}\right) \hat{n} \cdot \vec{v}_1 \\
& \hat{n} \cdot \vec{v}_2 \hat{n} \times \vec{S}_1 \cdot \vec{v}_2 + 72 \log\left(\frac{r}{R_\theta}\right) \vec{v}_1 \cdot \vec{v}_2 \hat{n} \times \vec{S}_1 \cdot \vec{v}_2 + 72 \log\left(\frac{r}{R_\theta}\right) \vec{v}_2 \cdot \vec{v}_2 \hat{n} \times \vec{S}_1 \cdot \vec{v}_2 + 192 (\hat{n} \cdot \vec{v}_2)^2 \hat{n} \times \vec{S}_1 \cdot \vec{v}_2 + \\
& \left. 24 \hat{n} \cdot \vec{v}_2 \vec{S}_1 \times \vec{v}_1 \cdot \vec{v}_2 + 192 \hat{n} \cdot \vec{v}_1 \hat{n} \cdot \vec{v}_2 \hat{n} \times \vec{S}_1 \cdot \vec{v}_2 - 24 \vec{v}_1 \cdot \vec{v}_2 \hat{n} \times \vec{S}_1 \cdot \vec{v}_2 - \frac{152}{5} \vec{v}_2 \cdot \vec{v}_2 \hat{n} \times \vec{S}_1 \cdot \vec{v}_2 \right) \Big\}
\end{aligned}$$

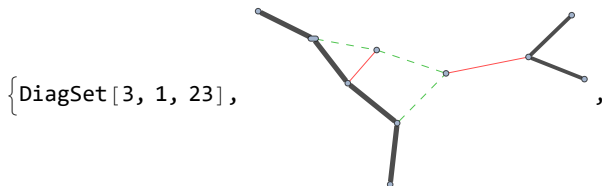

$$\frac{32 G^3 m_1^2 m_2 \vec{S}_1 \times \vec{v}_1 \cdot \vec{a}_1}{3 r^3} + \frac{G^3 m_1^2 m_2 \left( \frac{68}{5} \vec{v}_1 \cdot \vec{v}_1 \hat{n} \times \vec{S}_1 \cdot \vec{v}_1 + \frac{12}{5} \vec{v}_2 \cdot \vec{v}_2 \hat{n} \times \vec{S}_1 \cdot \vec{v}_1 \right)}{r^4} \Big\}$$

$\{\text{DiagSet}[3, 1, 24],$  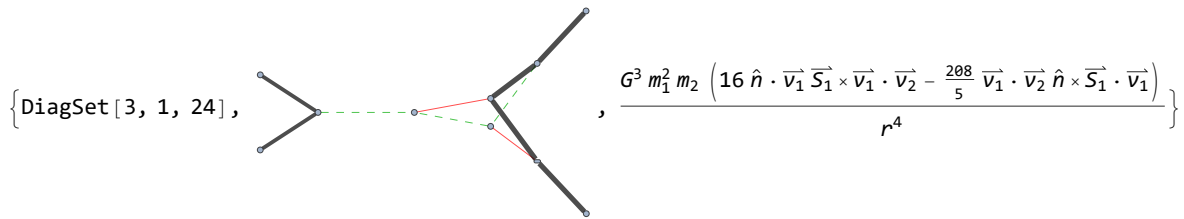 ,  $\frac{G^3 m_1^2 m_2 \left( 16 \hat{n} \cdot \vec{v}_1 \vec{S}_1 \times \vec{v}_1 \cdot \vec{v}_2 - \frac{208}{5} \vec{v}_1 \cdot \vec{v}_2 \hat{n} \times \vec{S}_1 \cdot \vec{v}_1 \right)}{r^4} \}$

$\{\text{DiagSet}[3, 1, 25],$  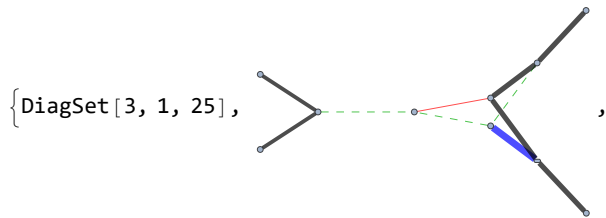 ,

$\frac{G^3 m_1^2 m_2 \left( -\frac{12}{5} \hat{n} \cdot \vec{v}_1 \vec{S}_1 \times \vec{v}_1 \cdot \vec{v}_2 - \frac{72}{5} \vec{v}_1 \cdot \vec{v}_1 \hat{n} \times \vec{S}_1 \cdot \vec{v}_2 + \frac{108}{5} \vec{v}_1 \cdot \vec{v}_2 \hat{n} \times \vec{S}_1 \cdot \vec{v}_1 \right)}{r^4} \}$

$\{\text{DiagSet}[3, 1, 26],$  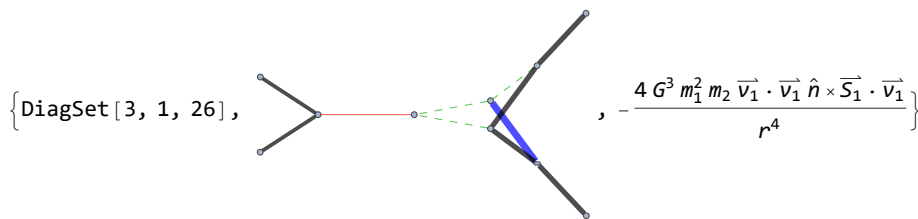 ,  $-\frac{4 G^3 m_1^2 m_2 \vec{v}_1 \cdot \vec{v}_1 \hat{n} \times \vec{S}_1 \cdot \vec{v}_1}{r^4} \}$

$\{\text{DiagSet}[3, 1, 27],$  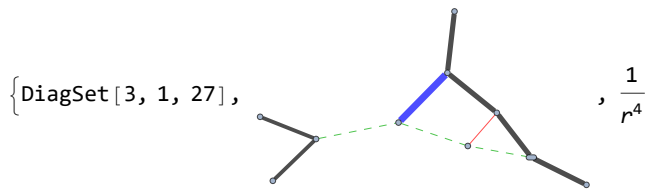 ,  $\frac{1}{r^4}$

$G^3 m_1^2 m_2 \left( \frac{-16 (\hat{n} \cdot \vec{v}_1)^2 \hat{n} \times \vec{S}_1 \cdot \vec{v}_2 - \frac{32}{5} \hat{n} \cdot \vec{v}_1 \vec{S}_1 \times \vec{v}_1 \cdot \vec{v}_2 + \frac{16}{5} \vec{v}_1 \cdot \vec{v}_1 \hat{n} \times \vec{S}_1 \cdot \vec{v}_2}{\epsilon_d} + \right.$   
 $48 \log\left(\frac{r}{R_0}\right) (\hat{n} \cdot \vec{v}_1)^2 \hat{n} \times \vec{S}_1 \cdot \vec{v}_2 + \frac{96}{5} \log\left(\frac{r}{R_0}\right) \hat{n} \cdot \vec{v}_1 \vec{S}_1 \times \vec{v}_1 \cdot \vec{v}_2 - \frac{48}{5} \log\left(\frac{r}{R_0}\right) \vec{v}_1 \cdot \vec{v}_1 \hat{n} \times \vec{S}_1 \cdot \vec{v}_2 -$   
 $\left. 32 (\hat{n} \cdot \vec{v}_1)^2 \hat{n} \times \vec{S}_1 \cdot \vec{v}_2 - \frac{264}{25} \hat{n} \cdot \vec{v}_1 \vec{S}_1 \times \vec{v}_1 \cdot \vec{v}_2 + \frac{232}{25} \vec{v}_1 \cdot \vec{v}_1 \hat{n} \times \vec{S}_1 \cdot \vec{v}_2 - \frac{24}{5} \vec{v}_1 \cdot \vec{v}_2 \hat{n} \times \vec{S}_1 \cdot \vec{v}_1 \right) \}$

$\{\text{DiagSet}[3, 1, 28],$  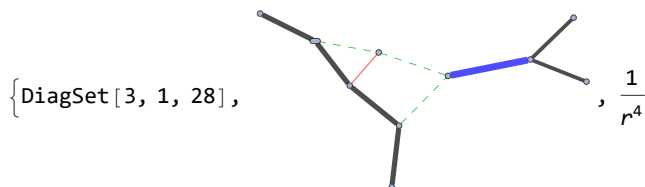 ,  $\frac{1}{r^4}$

$G^3 m_1^2 m_2 \left( \frac{\frac{16}{7} (\hat{n} \cdot \vec{v}_2)^2 \hat{n} \times \vec{S}_1 \cdot \vec{v}_1 - \frac{32}{35} \hat{n} \cdot \vec{v}_2 \vec{S}_1 \times \vec{v}_1 \cdot \vec{v}_2 - \frac{16}{35} \vec{v}_2 \cdot \vec{v}_2 \hat{n} \times \vec{S}_1 \cdot \vec{v}_1}{\epsilon_d} - \right.$   
 $\frac{48}{7} \log\left(\frac{r}{R_0}\right) (\hat{n} \cdot \vec{v}_2)^2 \hat{n} \times \vec{S}_1 \cdot \vec{v}_1 + \frac{96}{35} \log\left(\frac{r}{R_0}\right) \hat{n} \cdot \vec{v}_2 \vec{S}_1 \times \vec{v}_1 \cdot \vec{v}_2 + \frac{48}{35} \log\left(\frac{r}{R_0}\right) \vec{v}_2 \cdot \vec{v}_2 \hat{n} \times \vec{S}_1 \cdot \vec{v}_1 +$   
 $\left. \frac{288}{49} (\hat{n} \cdot \vec{v}_2)^2 \hat{n} \times \vec{S}_1 \cdot \vec{v}_1 - \frac{3048 \hat{n} \cdot \vec{v}_2 \vec{S}_1 \times \vec{v}_1 \cdot \vec{v}_2}{1225} + \frac{8}{5} \vec{v}_1 \cdot \vec{v}_2 \hat{n} \times \vec{S}_1 \cdot \vec{v}_2 - \frac{2504 \vec{v}_2 \cdot \vec{v}_2 \hat{n} \times \vec{S}_1 \cdot \vec{v}_1}{1225} \right) \}$

{DiagSet[3, 1, 29],

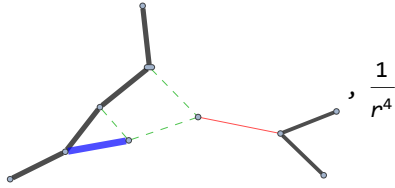

,  $\frac{1}{r^4}$

$$G^3 m_1^2 m_2 \left( \frac{\frac{64}{35} \vec{v}_1 \cdot \vec{v}_1 \hat{n} \times \vec{S}_1 \cdot \vec{v}_1 - \frac{64}{7} (\hat{n} \cdot \vec{v}_1)^2 \hat{n} \times \vec{S}_1 \cdot \vec{v}_1}{\epsilon_d} + \frac{192}{7} \log\left(\frac{r}{R_\theta}\right) (\hat{n} \cdot \vec{v}_1)^2 \hat{n} \times \vec{S}_1 \cdot \vec{v}_1 - \right.$$

$$\left. \frac{192}{35} \log\left(\frac{r}{R_\theta}\right) \vec{v}_1 \cdot \vec{v}_1 \hat{n} \times \vec{S}_1 \cdot \vec{v}_1 - \frac{1824}{49} (\hat{n} \cdot \vec{v}_1)^2 \hat{n} \times \vec{S}_1 \cdot \vec{v}_1 + \frac{9456 \vec{v}_1 \cdot \vec{v}_1 \hat{n} \times \vec{S}_1 \cdot \vec{v}_1}{1225} \right\}$$

{DiagSet[3, 1, 30],

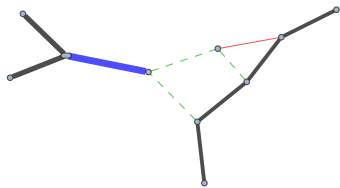

,  $\frac{G^3 m_2^3 \left( 32 \vec{v}_1 \cdot \vec{v}_2 \hat{n} \times \vec{S}_1 \cdot \vec{v}_2 - \frac{128}{5} \vec{v}_2 \cdot \vec{v}_2 \hat{n} \times \vec{S}_1 \cdot \vec{v}_1 \right)}{r^4}$

{DiagSet[3, 1, 31],

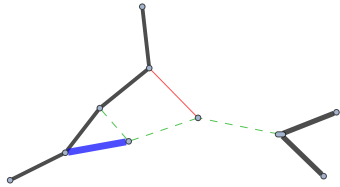

,  $\frac{G^3 m_2^3 \left( 128 (\hat{n} \cdot \vec{v}_2)^2 \hat{n} \times \vec{S}_1 \cdot \vec{v}_2 - 32 \vec{v}_2 \cdot \vec{v}_2 \hat{n} \times \vec{S}_1 \cdot \vec{v}_2 \right)}{r^4}$

{DiagSet[3, 1, 32],

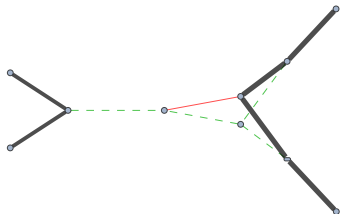

,

$$\frac{1}{r^3} m_1^2 m_2 \left( \frac{52}{5} \log\left(\frac{r}{R_\theta}\right) \vec{S}_1 \times \vec{v}_1 \cdot \vec{v}_2 + \frac{242}{25} \vec{S}_1 \times \vec{v}_1 \cdot \vec{v}_2 - 2 \vec{S}_1 \times \vec{a}_1 \cdot \vec{v}_2 - \frac{84}{25} \vec{S}_1 \times \vec{v}_1 \cdot \vec{a}_2 + \right.$$

$$\frac{134}{25} \hat{n} \times \vec{S}_1 \cdot \vec{v}_1 \hat{n} \cdot \vec{a}_2 + \frac{64}{25} \hat{n} \times \vec{S}_1 \cdot \vec{v}_2 \hat{n} \cdot \vec{v}_1 - \frac{78}{25} \hat{n} \times \vec{S}_1 \cdot \vec{a}_2 \hat{n} \cdot \vec{v}_1 - \frac{42}{25} \hat{n} \times \vec{S}_1 \cdot \vec{v}_1 \hat{n} \cdot \vec{v}_2 +$$

$$10 \hat{n} \times \vec{S}_1 \cdot \vec{a}_1 \hat{n} \cdot \vec{v}_2 + 12 \vec{S}_1 \times \vec{a}_1 \cdot \vec{v}_2 \log\left(\frac{r}{R_\theta}\right) - \frac{24}{5} \vec{S}_1 \times \vec{v}_1 \cdot \vec{a}_2 \log\left(\frac{r}{R_\theta}\right) - \frac{36}{5} \hat{n} \times \vec{S}_1 \cdot \vec{v}_1 \hat{n} \cdot \vec{a}_2 \log\left(\frac{r}{R_\theta}\right) +$$

$$\frac{144}{5} \hat{n} \times \vec{S}_1 \cdot \vec{v}_2 \hat{n} \cdot \vec{v}_1 \log\left(\frac{r}{R_\theta}\right) - \frac{108}{5} \hat{n} \times \vec{S}_1 \cdot \vec{a}_2 \hat{n} \cdot \vec{v}_1 \log\left(\frac{r}{R_\theta}\right) - \frac{12}{5} \hat{n} \times \vec{S}_1 \cdot \vec{v}_1 \hat{n} \cdot \vec{v}_2 \log\left(\frac{r}{R_\theta}\right) -$$

$$36 \hat{n} \times \vec{S}_1 \cdot \vec{a}_1 \hat{n} \cdot \vec{v}_2 \log\left(\frac{r}{R_\theta}\right) + \frac{1}{\epsilon_d} \left( -\frac{52}{15} \vec{S}_1 \times \vec{v}_1 \cdot \vec{v}_2 - 4 \vec{S}_1 \times \vec{a}_1 \cdot \vec{v}_2 + \frac{8}{5} \vec{S}_1 \times \vec{v}_1 \cdot \vec{a}_2 + \frac{12}{5} \hat{n} \times \vec{S}_1 \cdot \vec{v}_1 \hat{n} \cdot \vec{a}_2 - \right.$$

$$\left. \frac{48}{5} \hat{n} \times \vec{S}_1 \cdot \vec{v}_2 \hat{n} \cdot \vec{v}_1 + \frac{36}{5} \hat{n} \times \vec{S}_1 \cdot \vec{a}_2 \hat{n} \cdot \vec{v}_1 + \frac{4}{5} \hat{n} \times \vec{S}_1 \cdot \vec{v}_1 \hat{n} \cdot \vec{v}_2 + 12 \hat{n} \times \vec{S}_1 \cdot \vec{a}_1 \hat{n} \cdot \vec{v}_2 \right) \Big) G^3 +$$

$$\frac{1}{r^4} m_1^2 m_2 \left( -\frac{550}{49} \hat{n} \times \vec{S}_1 \cdot \vec{v}_2 (\hat{n} \cdot \vec{v}_1)^2 - \frac{396}{7} \hat{n} \times \vec{S}_1 \cdot \vec{v}_2 \log\left(\frac{r}{R_\theta}\right) (\hat{n} \cdot \vec{v}_1)^2 - \frac{15038 \vec{S}_1 \times \vec{v}_1 \cdot \vec{v}_2 \hat{n} \cdot \vec{v}_1}{1225} + \right.$$

$$\frac{670}{49} \hat{n} \times \vec{S}_1 \cdot \vec{v}_1 \hat{n} \cdot \vec{v}_2 \hat{n} \cdot \vec{v}_1 + 6 \hat{n} \times \vec{S}_1 \cdot \vec{v}_2 \hat{n} \cdot \vec{v}_2 \hat{n} \cdot \vec{v}_1 - \frac{804}{35} \vec{S}_1 \times \vec{v}_1 \cdot \vec{v}_2 \log\left(\frac{r}{R_\theta}\right) \hat{n} \cdot \vec{v}_1 +$$

$$\left. \frac{12}{7} \hat{n} \times \vec{S}_1 \cdot \vec{v}_1 \hat{n} \cdot \vec{v}_2 \log\left(\frac{r}{R_\theta}\right) \hat{n} \cdot \vec{v}_1 - 108 \hat{n} \times \vec{S}_1 \cdot \vec{v}_2 \hat{n} \cdot \vec{v}_2 \log\left(\frac{r}{R_\theta}\right) \hat{n} \cdot \vec{v}_1 + 34 \hat{n} \times \vec{S}_1 \cdot \vec{v}_1 (\hat{n} \cdot \vec{v}_2)^2 - \right.$$



$$\begin{aligned} & \frac{266}{25} \vec{S}_1 \times \vec{v}_1 \cdot \vec{v}_2 \hat{n} \cdot \vec{v}_2 + \frac{7202 \hat{n} \times \vec{S}_1 \cdot \vec{v}_2 \vec{v}_1 \cdot \vec{v}_1}{1225} - \frac{20234 \hat{n} \times \vec{S}_1 \cdot \vec{v}_1 \vec{v}_1 \cdot \vec{v}_2}{1225} + \frac{78}{25} \hat{n} \times \vec{S}_1 \cdot \vec{v}_2 \vec{v}_1 \cdot \vec{v}_2 - \\ & \frac{134}{25} \hat{n} \times \vec{S}_1 \cdot \vec{v}_1 \vec{v}_2 \cdot \vec{v}_2 - 36 \hat{n} \times \vec{S}_1 \cdot \vec{v}_1 (\hat{n} \cdot \vec{v}_2)^2 \log\left(\frac{r}{R_\theta}\right) - \frac{36}{5} \vec{S}_1 \times \vec{v}_1 \cdot \vec{v}_2 \hat{n} \cdot \vec{v}_2 \log\left(\frac{r}{R_\theta}\right) + \\ & \frac{396}{35} \hat{n} \times \vec{S}_1 \cdot \vec{v}_2 \vec{v}_1 \cdot \vec{v}_1 \log\left(\frac{r}{R_\theta}\right) - \frac{12}{35} \hat{n} \times \vec{S}_1 \cdot \vec{v}_1 \vec{v}_1 \cdot \vec{v}_2 \log\left(\frac{r}{R_\theta}\right) + \frac{108}{5} \hat{n} \times \vec{S}_1 \cdot \vec{v}_2 \vec{v}_1 \cdot \vec{v}_2 \log\left(\frac{r}{R_\theta}\right) + \\ & \frac{36}{5} \hat{n} \times \vec{S}_1 \cdot \vec{v}_1 \vec{v}_2 \cdot \vec{v}_2 \log\left(\frac{r}{R_\theta}\right) + \frac{1}{\epsilon_d} \left( \frac{132}{7} \hat{n} \times \vec{S}_1 \cdot \vec{v}_2 (\hat{n} \cdot \vec{v}_1)^2 + \frac{268}{35} \vec{S}_1 \times \vec{v}_1 \cdot \vec{v}_2 \hat{n} \cdot \vec{v}_1 - \right. \\ & \left. \frac{4}{7} \hat{n} \times \vec{S}_1 \cdot \vec{v}_1 \hat{n} \cdot \vec{v}_2 \hat{n} \cdot \vec{v}_1 + 36 \hat{n} \times \vec{S}_1 \cdot \vec{v}_2 \hat{n} \cdot \vec{v}_2 \hat{n} \cdot \vec{v}_1 + 12 \hat{n} \times \vec{S}_1 \cdot \vec{v}_1 (\hat{n} \cdot \vec{v}_2)^2 + \frac{12}{5} \vec{S}_1 \times \vec{v}_1 \cdot \vec{v}_2 \hat{n} \cdot \vec{v}_2 - \right. \\ & \left. \frac{132}{35} \hat{n} \times \vec{S}_1 \cdot \vec{v}_2 \vec{v}_1 \cdot \vec{v}_1 + \frac{4}{35} \hat{n} \times \vec{S}_1 \cdot \vec{v}_1 \vec{v}_1 \cdot \vec{v}_2 - \frac{36}{5} \hat{n} \times \vec{S}_1 \cdot \vec{v}_2 \vec{v}_1 \cdot \vec{v}_2 - \frac{12}{5} \hat{n} \times \vec{S}_1 \cdot \vec{v}_1 \vec{v}_2 \cdot \vec{v}_2 \right) \Bigg) G^3 \Bigg\} \end{aligned}$$

{DiagSet[3, 1, 33], 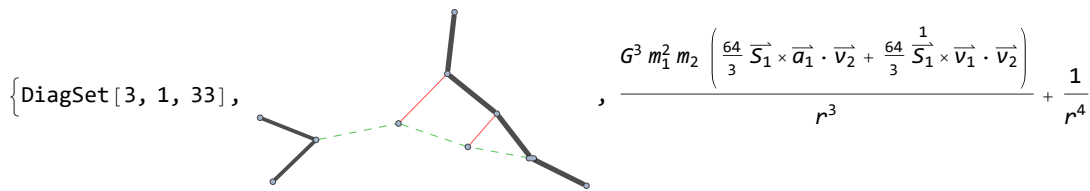

$$, \frac{G^3 m_1^2 m_2 \left( \frac{64}{3} \vec{S}_1 \times \vec{a}_1 \cdot \vec{v}_2 + \frac{64}{3} \vec{S}_1 \times \vec{v}_1 \cdot \vec{v}_2 \right)}{r^3} + \frac{1}{r^4}$$

{DiagSet[3, 1, 34], 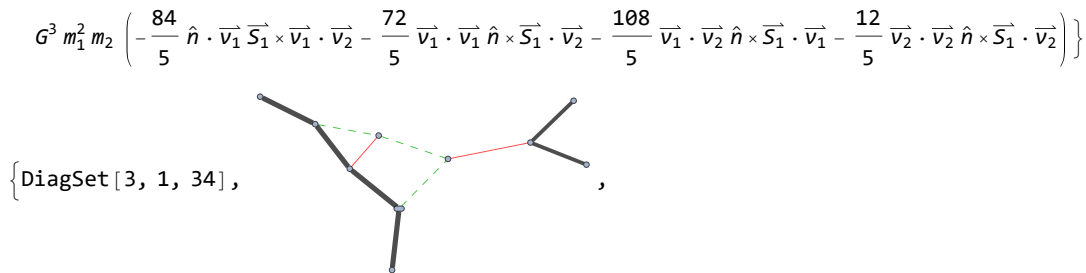

$$, \frac{G^3 m_1^2 m_2 \left( -\frac{84}{5} \hat{n} \cdot \vec{v}_1 \vec{S}_1 \times \vec{v}_1 \cdot \vec{v}_2 - \frac{72}{5} \vec{v}_1 \cdot \vec{v}_1 \hat{n} \times \vec{S}_1 \cdot \vec{v}_2 - \frac{108}{5} \vec{v}_1 \cdot \vec{v}_2 \hat{n} \times \vec{S}_1 \cdot \vec{v}_1 - \frac{12}{5} \vec{v}_2 \cdot \vec{v}_2 \hat{n} \times \vec{S}_1 \cdot \vec{v}_2 \right)}{r^4} \Bigg\}$$

{DiagSet[3, 1, 35], 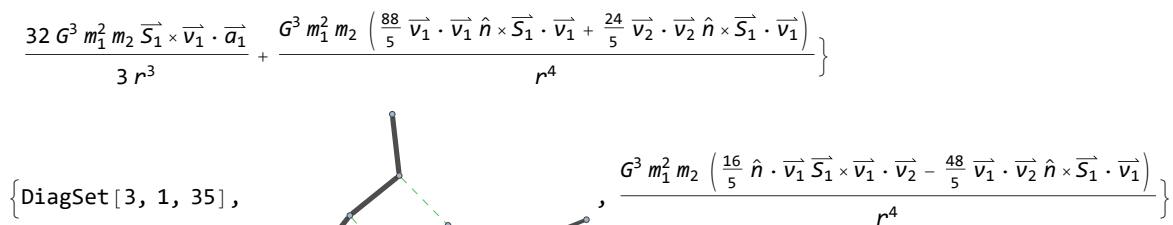

$$, \frac{G^3 m_1^2 m_2 \left( \frac{16}{5} \hat{n} \cdot \vec{v}_1 \vec{S}_1 \times \vec{v}_1 \cdot \vec{v}_2 - \frac{48}{5} \vec{v}_1 \cdot \vec{v}_2 \hat{n} \times \vec{S}_1 \cdot \vec{v}_1 \right)}{r^4} \Bigg\}$$

{DiagSet[3, 1, 36], 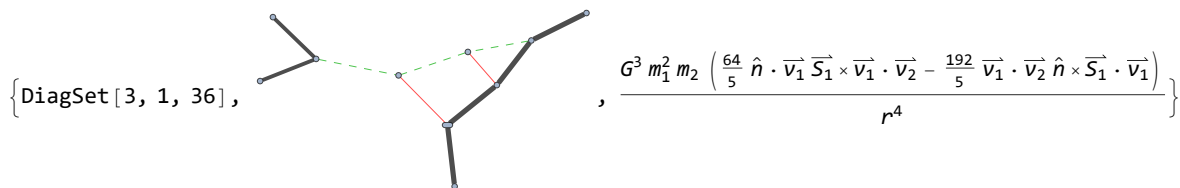

$$, \frac{G^3 m_1^2 m_2 \left( \frac{64}{5} \hat{n} \cdot \vec{v}_1 \vec{S}_1 \times \vec{v}_1 \cdot \vec{v}_2 - \frac{192}{5} \vec{v}_1 \cdot \vec{v}_2 \hat{n} \times \vec{S}_1 \cdot \vec{v}_1 \right)}{r^4} \Bigg\}$$

{DiagSet[3, 1, 37], 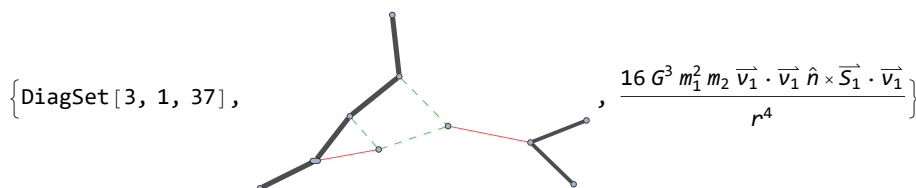

$$, \frac{16 G^3 m_1^2 m_2 \vec{v}_1 \cdot \vec{v}_1 \hat{n} \times \vec{S}_1 \cdot \vec{v}_1}{r^4} \Bigg\}$$

$\{ \text{DiagSet}[3, 1, 38],$ 
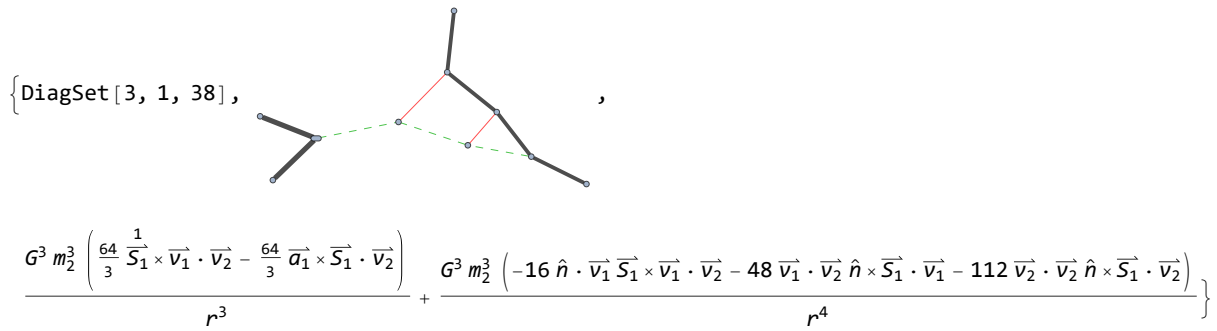
 $,$ 

$$\frac{G^3 m_2^3 \left( \frac{64}{3} \vec{S}_1 \times \vec{v}_1 \cdot \vec{v}_2 - \frac{64}{3} \vec{a}_1 \times \vec{S}_1 \cdot \vec{v}_2 \right)}{r^3} + \frac{G^3 m_2^3 \left( -16 \hat{n} \cdot \vec{v}_1 \vec{S}_1 \times \vec{v}_1 \cdot \vec{v}_2 - 48 \vec{v}_1 \cdot \vec{v}_2 \hat{n} \times \vec{S}_1 \cdot \vec{v}_1 - 112 \vec{v}_2 \cdot \vec{v}_2 \hat{n} \times \vec{S}_1 \cdot \vec{v}_2 \right)}{r^4} \}$$

$\{ \text{DiagSet}[3, 1, 39],$ 
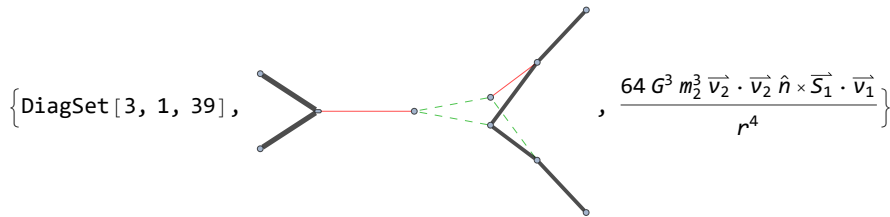
 $, \frac{64 G^3 m_2^3 \vec{v}_2 \cdot \vec{v}_2 \hat{n} \times \vec{S}_1 \cdot \vec{v}_1}{r^4} \}$

$\{ \text{DiagSet}[3, 1, 40],$ 
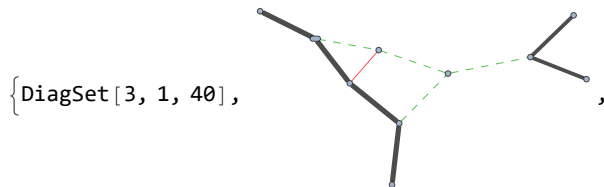
 $,$

$$\begin{aligned}
 & \frac{1}{r^3} m_1^2 m_2 \left( \frac{24}{5} \log\left(\frac{r}{R_\theta}\right) \vec{S}_1 \times \vec{v}_1 \cdot \vec{v}_2 - \frac{16}{25} \vec{S}_1 \times \vec{v}_1 \cdot \vec{v}_2 - \frac{52}{75} \vec{S}_1 \times \vec{a}_1 \cdot \vec{v}_2 + \frac{52}{75} \vec{S}_1 \times \vec{v}_1 \cdot \vec{a}_2 - 6 \hat{n} \times \vec{S}_1 \cdot \vec{v}_2 \hat{n} \cdot \vec{v}_1 + \right. \\
 & \frac{112}{25} \hat{n} \times \vec{S}_1 \cdot \vec{a}_2 \hat{n} \cdot \vec{v}_1 + \frac{38}{25} \hat{n} \times \vec{S}_1 \cdot \vec{v}_1 \hat{n} \cdot \vec{v}_2 + \frac{112}{25} \hat{n} \times \vec{S}_1 \cdot \vec{a}_1 \hat{n} \cdot \vec{v}_2 + \frac{16}{5} \vec{S}_1 \times \vec{a}_1 \cdot \vec{v}_2 \log\left(\frac{r}{R_\theta}\right) - \\
 & \frac{16}{5} \vec{S}_1 \times \vec{v}_1 \cdot \vec{a}_2 \log\left(\frac{r}{R_\theta}\right) + 12 \hat{n} \times \vec{S}_1 \cdot \vec{v}_2 \hat{n} \cdot \vec{v}_1 \log\left(\frac{r}{R_\theta}\right) - \frac{48}{5} \hat{n} \times \vec{S}_1 \cdot \vec{a}_2 \hat{n} \cdot \vec{v}_1 \log\left(\frac{r}{R_\theta}\right) - \\
 & \frac{12}{5} \hat{n} \times \vec{S}_1 \cdot \vec{v}_1 \hat{n} \cdot \vec{v}_2 \log\left(\frac{r}{R_\theta}\right) - \frac{48}{5} \hat{n} \times \vec{S}_1 \cdot \vec{a}_1 \hat{n} \cdot \vec{v}_2 \log\left(\frac{r}{R_\theta}\right) + \frac{1}{\epsilon_d} \left( -\frac{8}{5} \vec{S}_1 \times \vec{v}_1 \cdot \vec{v}_2 - \frac{16}{15} \vec{S}_1 \times \vec{a}_1 \cdot \vec{v}_2 + \right. \\
 & \left. \frac{16}{15} \vec{S}_1 \times \vec{v}_1 \cdot \vec{a}_2 - 4 \hat{n} \times \vec{S}_1 \cdot \vec{v}_2 \hat{n} \cdot \vec{v}_1 + \frac{16}{5} \hat{n} \times \vec{S}_1 \cdot \vec{a}_2 \hat{n} \cdot \vec{v}_1 + \frac{4}{5} \hat{n} \times \vec{S}_1 \cdot \vec{v}_1 \hat{n} \cdot \vec{v}_2 + \frac{16}{5} \hat{n} \times \vec{S}_1 \cdot \vec{a}_1 \hat{n} \cdot \vec{v}_2 \right) \Big) G^3 + \\
 & \frac{1}{r^4} m_1^2 m_2 \left( 32 \hat{n} \times \vec{S}_1 \cdot \vec{v}_2 (\hat{n} \cdot \vec{v}_1)^2 - 48 \hat{n} \times \vec{S}_1 \cdot \vec{v}_2 \log\left(\frac{r}{R_\theta}\right) (\hat{n} \cdot \vec{v}_1)^2 + \frac{14024 \vec{S}_1 \times \vec{v}_1 \cdot \vec{v}_2 \hat{n} \cdot \vec{v}_1}{1225} - \right. \\
 & \frac{576}{49} \hat{n} \times \vec{S}_1 \cdot \vec{v}_1 \hat{n} \cdot \vec{v}_2 \hat{n} \cdot \vec{v}_1 + 32 \hat{n} \times \vec{S}_1 \cdot \vec{v}_2 \hat{n} \cdot \vec{v}_2 \hat{n} \cdot \vec{v}_1 - \frac{768}{35} \vec{S}_1 \times \vec{v}_1 \cdot \vec{v}_2 \log\left(\frac{r}{R_\theta}\right) \hat{n} \cdot \vec{v}_1 + \\
 & \frac{96}{7} \hat{n} \times \vec{S}_1 \cdot \vec{v}_1 \hat{n} \cdot \vec{v}_2 \log\left(\frac{r}{R_\theta}\right) \hat{n} \cdot \vec{v}_1 - 48 \hat{n} \times \vec{S}_1 \cdot \vec{v}_2 \hat{n} \cdot \vec{v}_2 \log\left(\frac{r}{R_\theta}\right) \hat{n} \cdot \vec{v}_1 + \frac{132}{25} \vec{S}_1 \times \vec{v}_1 \cdot \vec{v}_2 \hat{n} \cdot \vec{v}_2 - \\
 & \frac{112}{25} \hat{n} \times \vec{S}_1 \cdot \vec{v}_2 \vec{v}_1 \cdot \vec{v}_1 + \frac{108 \hat{n} \times \vec{S}_1 \cdot \vec{v}_1 \vec{v}_1 \cdot \vec{v}_2}{1225} - \frac{112}{25} \hat{n} \times \vec{S}_1 \cdot \vec{v}_2 \vec{v}_1 \cdot \vec{v}_2 - \frac{48}{5} \vec{S}_1 \times \vec{v}_1 \cdot \vec{v}_2 \hat{n} \cdot \vec{v}_2 \log\left(\frac{r}{R_\theta}\right) + \\
 & \frac{48}{5} \hat{n} \times \vec{S}_1 \cdot \vec{v}_2 \vec{v}_1 \cdot \vec{v}_1 \log\left(\frac{r}{R_\theta}\right) - \frac{96}{35} \hat{n} \times \vec{S}_1 \cdot \vec{v}_1 \vec{v}_1 \cdot \vec{v}_2 \log\left(\frac{r}{R_\theta}\right) + \frac{48}{5} \hat{n} \times \vec{S}_1 \cdot \vec{v}_2 \vec{v}_1 \cdot \vec{v}_2 \log\left(\frac{r}{R_\theta}\right) + \frac{1}{\epsilon_d} \\
 & \left( 16 \hat{n} \times \vec{S}_1 \cdot \vec{v}_2 (\hat{n} \cdot \vec{v}_1)^2 + \frac{256}{35} \vec{S}_1 \times \vec{v}_1 \cdot \vec{v}_2 \hat{n} \cdot \vec{v}_1 - \frac{32}{7} \hat{n} \times \vec{S}_1 \cdot \vec{v}_1 \hat{n} \cdot \vec{v}_2 \hat{n} \cdot \vec{v}_1 + 16 \hat{n} \times \vec{S}_1 \cdot \vec{v}_2 \hat{n} \cdot \vec{v}_2 \hat{n} \cdot \vec{v}_1 + \right. \\
 & \left. \frac{16}{5} \vec{S}_1 \times \vec{v}_1 \cdot \vec{v}_2 \hat{n} \cdot \vec{v}_2 - \frac{16}{5} \hat{n} \times \vec{S}_1 \cdot \vec{v}_2 \vec{v}_1 \cdot \vec{v}_1 + \frac{32}{35} \hat{n} \times \vec{S}_1 \cdot \vec{v}_1 \vec{v}_1 \cdot \vec{v}_2 - \frac{16}{5} \hat{n} \times \vec{S}_1 \cdot \vec{v}_2 \vec{v}_1 \cdot \vec{v}_2 \right) \Big) G^3 \}
 \end{aligned}$$

{DiagSet[3, 1, 41],

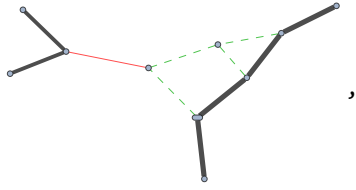

,

$$\frac{1}{r^3} G^3 m_1^2 m_2 \left( \frac{-\frac{48}{5} \hat{n} \cdot \vec{a}_1 \hat{n} \times \vec{S}_1 \cdot \vec{v}_1 + \frac{16}{5} \hat{n} \cdot \vec{v}_1 \hat{n} \times \vec{S}_1 \cdot \vec{a}_1 + \frac{64}{15} \vec{S}_1 \times \vec{v}_1 \cdot \vec{a}_1 + \frac{16}{5} \hat{n} \cdot \vec{v}_1 \hat{n} \times \vec{S}_1 \cdot \vec{v}_1}{\epsilon_d} + \right.$$

$$\frac{144}{5} \log\left(\frac{r}{R_\theta}\right) \hat{n} \cdot \vec{a}_1 \hat{n} \times \vec{S}_1 \cdot \vec{v}_1 - \frac{48}{5} \log\left(\frac{r}{R_\theta}\right) \hat{n} \cdot \vec{v}_1 \hat{n} \times \vec{S}_1 \cdot \vec{a}_1 - \frac{416}{25} \hat{n} \cdot \vec{a}_1 \hat{n} \times \vec{S}_1 \cdot \vec{v}_1 - \frac{128}{25} \hat{n} \cdot \vec{v}_1 \hat{n} \times \vec{S}_1 \cdot \vec{a}_1 -$$

$$\left. \frac{64}{5} \log\left(\frac{r}{R_\theta}\right) \vec{S}_1 \times \vec{v}_1 \cdot \vec{a}_1 + \frac{448}{75} \vec{S}_1 \times \vec{v}_1 \cdot \vec{a}_1 - \frac{48}{5} \log\left(\frac{r}{R_\theta}\right) \hat{n} \cdot \vec{v}_1 \hat{n} \times \vec{S}_1 \cdot \vec{v}_1 + \frac{272}{25} \hat{n} \cdot \vec{v}_1 \hat{n} \times \vec{S}_1 \cdot \vec{v}_1 \right) + \frac{1}{r^4}$$

$$G^3 m_1^2 m_2 \left( \frac{1}{\epsilon_d} \left( \frac{16}{7} (\hat{n} \cdot \vec{v}_1)^2 \hat{n} \times \vec{S}_1 \cdot \vec{v}_1 - \frac{16}{5} \hat{n} \cdot \vec{v}_1 \vec{S}_1 \times \vec{v}_1 \cdot \vec{v}_2 + 16 \hat{n} \cdot \vec{v}_2 \hat{n} \cdot \vec{v}_1 \hat{n} \times \vec{S}_1 \cdot \vec{v}_1 - \frac{16}{35} \vec{v}_1 \cdot \vec{v}_1 \hat{n} \times \vec{S}_1 \cdot \vec{v}_1 - \right. \right.$$

$$\frac{16}{5} \vec{v}_1 \cdot \vec{v}_2 \hat{n} \times \vec{S}_1 \cdot \vec{v}_1 \left. \right) - \frac{48}{7} \log\left(\frac{r}{R_\theta}\right) (\hat{n} \cdot \vec{v}_1)^2 \hat{n} \times \vec{S}_1 \cdot \vec{v}_1 + \frac{48}{5} \log\left(\frac{r}{R_\theta}\right) \hat{n} \cdot \vec{v}_1 \vec{S}_1 \times \vec{v}_1 \cdot \vec{v}_2 - 48 \log\left(\frac{r}{R_\theta}\right) \hat{n} \cdot \vec{v}_2$$

$$\hat{n} \cdot \vec{v}_1 \hat{n} \times \vec{S}_1 \cdot \vec{v}_1 + \frac{48}{35} \log\left(\frac{r}{R_\theta}\right) \vec{v}_1 \cdot \vec{v}_1 \hat{n} \times \vec{S}_1 \cdot \vec{v}_1 + \frac{48}{5} \log\left(\frac{r}{R_\theta}\right) \vec{v}_1 \cdot \vec{v}_2 \hat{n} \times \vec{S}_1 \cdot \vec{v}_1 + \frac{512}{49} (\hat{n} \cdot \vec{v}_1)^2 \hat{n} \times \vec{S}_1 \cdot \vec{v}_1 -$$

$$\left. \frac{272}{25} \hat{n} \cdot \vec{v}_1 \vec{S}_1 \times \vec{v}_1 \cdot \vec{v}_2 + 64 \hat{n} \cdot \vec{v}_2 \hat{n} \cdot \vec{v}_1 \hat{n} \times \vec{S}_1 \cdot \vec{v}_1 - \frac{4604 \vec{v}_1 \cdot \vec{v}_1 \hat{n} \times \vec{S}_1 \cdot \vec{v}_1}{1225} - \frac{272}{25} \vec{v}_1 \cdot \vec{v}_2 \hat{n} \times \vec{S}_1 \cdot \vec{v}_1 \right) \}$$

{DiagSet[3, 1, 42],

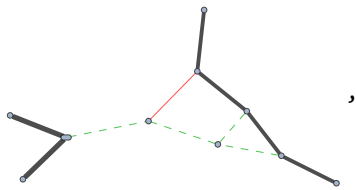

,

$$\frac{1}{r^3} G^3 m_2^3 \left( \frac{-16 \hat{n} \cdot \vec{a}_2 \hat{n} \times \vec{S}_1 \cdot \vec{v}_2 - 16 \hat{n} \cdot \vec{v}_2 \hat{n} \times \vec{a}_2 \cdot \vec{S}_1 + \frac{32}{3} \vec{a}_2 \times \vec{S}_1 \cdot \vec{v}_2}{\epsilon_d} + \right.$$

$$48 \log\left(\frac{r}{R_\theta}\right) \hat{n} \cdot \vec{a}_2 \hat{n} \times \vec{S}_1 \cdot \vec{v}_2 + 48 \log\left(\frac{r}{R_\theta}\right) \hat{n} \cdot \vec{v}_2 \hat{n} \times \vec{a}_2 \cdot \vec{S}_1 - 32 \hat{n} \cdot \vec{a}_2 \hat{n} \times \vec{S}_1 \cdot \vec{v}_2 +$$

$$\left. 32 \hat{n} \cdot \vec{v}_2 \hat{n} \times \vec{a}_2 \cdot \vec{S}_1 - 32 \log\left(\frac{r}{R_\theta}\right) \vec{a}_2 \times \vec{S}_1 \cdot \vec{v}_2 - \frac{32}{3} \vec{a}_2 \times \vec{S}_1 \cdot \vec{v}_2 + 32 \hat{n} \cdot \vec{v}_2 \hat{n} \times \vec{S}_1 \cdot \vec{v}_2 \right) +$$

$$\frac{1}{r^4} G^3 m_2^3 \left( -96 (\hat{n} \cdot \vec{v}_2)^2 \hat{n} \times \vec{S}_1 \cdot \vec{v}_2 - 32 \hat{n} \cdot \vec{v}_2 \vec{S}_1 \times \vec{v}_1 \cdot \vec{v}_2 - 160 \hat{n} \cdot \vec{v}_1 \hat{n} \cdot \vec{v}_2 \hat{n} \times \vec{S}_1 \cdot \vec{v}_2 + \right.$$

$$\left. 32 \vec{v}_1 \cdot \vec{v}_2 \hat{n} \times \vec{S}_1 \cdot \vec{v}_2 + 24 \vec{v}_2 \cdot \vec{v}_2 \hat{n} \times \vec{S}_1 \cdot \vec{v}_2 \right) \}$$

{DiagSet[3, 1, 43],

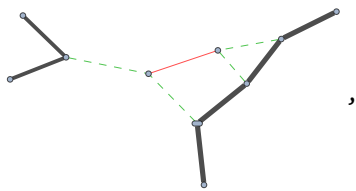

,

$$-\frac{32 G^3 m_1^2 m_2 \vec{v}_1 \cdot \vec{v}_1 \hat{n} \times \vec{S}_1 \cdot \vec{v}_2}{5 r^4} \}$$

$\left\{ \text{DiagSet}[3, 1, 44], \right.$ 
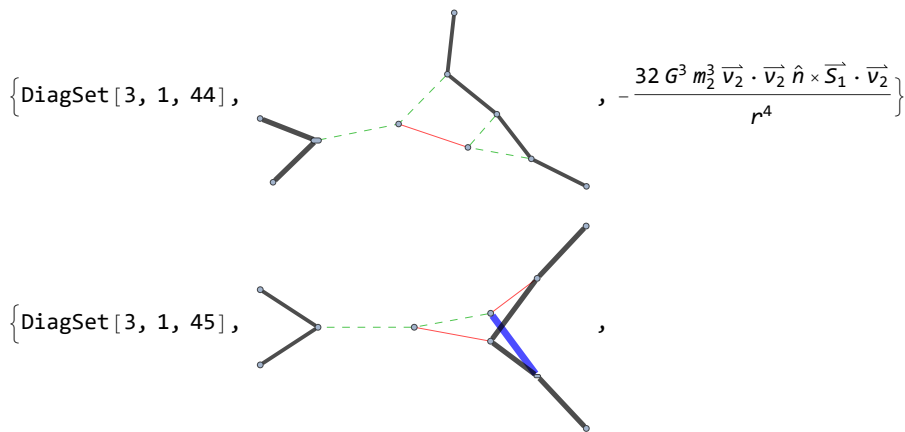
 $\left. , -\frac{32 G^3 m_2^3 \vec{v}_2 \cdot \vec{v}_2 \hat{n} \times \vec{S}_1 \cdot \vec{v}_2}{r^4} \right\}$

$\left\{ \text{DiagSet}[3, 1, 45], \right.$ 
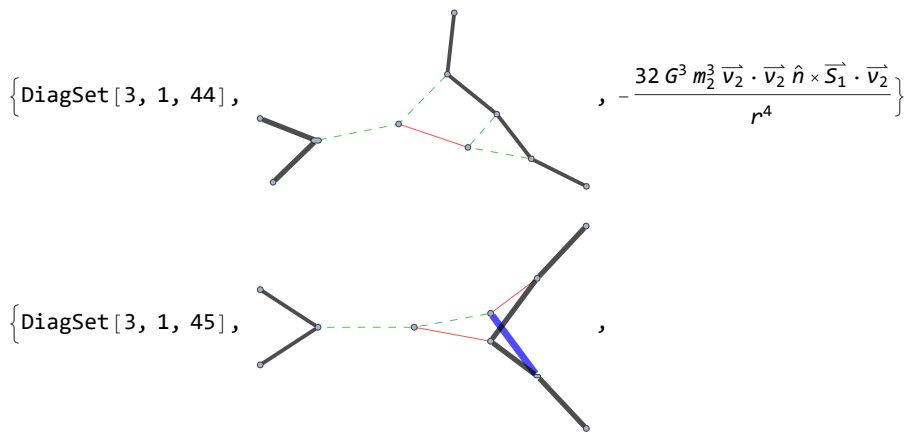
 $\left. , \right.$

$$\begin{aligned}
 & \frac{1}{r^3} m_1^2 m_2 \left( \frac{8}{5} \log\left(\frac{r}{R_\theta}\right) \vec{S}_1 \times \vec{v}_1 \cdot \vec{a}_2 + \frac{108}{25} \vec{S}_1 \times \vec{v}_1 \cdot \vec{a}_2 - \frac{58}{25} \hat{n} \times \vec{S}_1 \cdot \vec{v}_1 \hat{n} \cdot \vec{a}_2 - \frac{14}{25} \hat{n} \times \vec{S}_1 \cdot \vec{a}_2 \hat{n} \cdot \vec{v}_1 + \frac{12}{5} \hat{n} \times \vec{S}_1 \cdot \vec{v}_1 \hat{n} \cdot \vec{a}_2 \right. \\
 & \left. \log\left(\frac{r}{R_\theta}\right) + \frac{36}{5} \hat{n} \times \vec{S}_1 \cdot \vec{a}_2 \hat{n} \cdot \vec{v}_1 \log\left(\frac{r}{R_\theta}\right) + \frac{-\frac{8}{15} \vec{S}_1 \times \vec{v}_1 \cdot \vec{a}_2 - \frac{4}{5} \hat{n} \times \vec{S}_1 \cdot \vec{v}_1 \hat{n} \cdot \vec{a}_2 - \frac{12}{5} \hat{n} \times \vec{S}_1 \cdot \vec{a}_2 \hat{n} \cdot \vec{v}_1}{\epsilon_d} \right) G^3 + \frac{1}{r^4} \\
 & m_1^2 m_2 \left( 10 \hat{n} \times \vec{S}_1 \cdot \vec{v}_2 (\hat{n} \cdot \vec{v}_1)^2 - 36 \hat{n} \times \vec{S}_1 \cdot \vec{v}_2 \log\left(\frac{r}{R_\theta}\right) (\hat{n} \cdot \vec{v}_1)^2 - \frac{58}{5} \vec{S}_1 \times \vec{v}_1 \cdot \vec{v}_2 \hat{n} \cdot \vec{v}_1 + 14 \hat{n} \times \vec{S}_1 \cdot \vec{v}_1 \hat{n} \cdot \vec{v}_2 \hat{n} \cdot \vec{v}_1 - \right. \\
 & 10 \hat{n} \times \vec{S}_1 \cdot \vec{v}_2 \hat{n} \cdot \vec{v}_2 \hat{n} \cdot \vec{v}_1 - 12 \vec{S}_1 \times \vec{v}_1 \cdot \vec{v}_2 \log\left(\frac{r}{R_\theta}\right) \hat{n} \cdot \vec{v}_1 - 12 \hat{n} \times \vec{S}_1 \cdot \vec{v}_1 \hat{n} \cdot \vec{v}_2 \log\left(\frac{r}{R_\theta}\right) \hat{n} \cdot \vec{v}_1 + \\
 & 36 \hat{n} \times \vec{S}_1 \cdot \vec{v}_2 \hat{n} \cdot \vec{v}_2 \log\left(\frac{r}{R_\theta}\right) \hat{n} \cdot \vec{v}_1 - 14 \hat{n} \times \vec{S}_1 \cdot \vec{v}_1 (\hat{n} \cdot \vec{v}_2)^2 + \frac{342}{25} \vec{S}_1 \times \vec{v}_1 \cdot \vec{v}_2 \hat{n} \cdot \vec{v}_2 - \frac{14}{25} \hat{n} \times \vec{S}_1 \cdot \vec{v}_2 \vec{v}_1 \cdot \vec{v}_1 - \\
 & \frac{198}{25} \hat{n} \times \vec{S}_1 \cdot \vec{v}_1 \vec{v}_1 \cdot \vec{v}_2 + \frac{14}{25} \hat{n} \times \vec{S}_1 \cdot \vec{v}_2 \vec{v}_1 \cdot \vec{v}_2 + \frac{58}{25} \hat{n} \times \vec{S}_1 \cdot \vec{v}_1 \vec{v}_2 \cdot \vec{v}_2 + 12 \hat{n} \times \vec{S}_1 \cdot \vec{v}_1 (\hat{n} \cdot \vec{v}_2)^2 \log\left(\frac{r}{R_\theta}\right) + \\
 & \frac{12}{5} \vec{S}_1 \times \vec{v}_1 \cdot \vec{v}_2 \hat{n} \cdot \vec{v}_2 \log\left(\frac{r}{R_\theta}\right) + \frac{36}{5} \hat{n} \times \vec{S}_1 \cdot \vec{v}_2 \vec{v}_1 \cdot \vec{v}_1 \log\left(\frac{r}{R_\theta}\right) + \frac{12}{5} \hat{n} \times \vec{S}_1 \cdot \vec{v}_1 \vec{v}_1 \cdot \vec{v}_2 \log\left(\frac{r}{R_\theta}\right) - \\
 & \frac{36}{5} \hat{n} \times \vec{S}_1 \cdot \vec{v}_2 \vec{v}_1 \cdot \vec{v}_2 \log\left(\frac{r}{R_\theta}\right) - \frac{12}{5} \hat{n} \times \vec{S}_1 \cdot \vec{v}_1 \vec{v}_2 \cdot \vec{v}_2 \log\left(\frac{r}{R_\theta}\right) + \frac{1}{\epsilon_d} \left( 12 \hat{n} \times \vec{S}_1 \cdot \vec{v}_2 (\hat{n} \cdot \vec{v}_1)^2 + 4 \vec{S}_1 \times \vec{v}_1 \cdot \vec{v}_2 \hat{n} \cdot \vec{v}_1 + \right. \\
 & 4 \hat{n} \times \vec{S}_1 \cdot \vec{v}_1 \hat{n} \cdot \vec{v}_2 \hat{n} \cdot \vec{v}_1 - 12 \hat{n} \times \vec{S}_1 \cdot \vec{v}_2 \hat{n} \cdot \vec{v}_2 \hat{n} \cdot \vec{v}_1 - 4 \hat{n} \times \vec{S}_1 \cdot \vec{v}_1 (\hat{n} \cdot \vec{v}_2)^2 - \frac{4}{5} \vec{S}_1 \times \vec{v}_1 \cdot \vec{v}_2 \hat{n} \cdot \vec{v}_2 - \\
 & \left. \left. \frac{12}{5} \hat{n} \times \vec{S}_1 \cdot \vec{v}_2 \vec{v}_1 \cdot \vec{v}_1 - \frac{4}{5} \hat{n} \times \vec{S}_1 \cdot \vec{v}_1 \vec{v}_1 \cdot \vec{v}_2 + \frac{12}{5} \hat{n} \times \vec{S}_1 \cdot \vec{v}_2 \vec{v}_1 \cdot \vec{v}_2 + \frac{4}{5} \hat{n} \times \vec{S}_1 \cdot \vec{v}_1 \vec{v}_2 \cdot \vec{v}_2 \right) \right) G^3 \Big\}
 \end{aligned}$$

$\left\{ \text{DiagSet}[3, 1, 46], \right.$ 
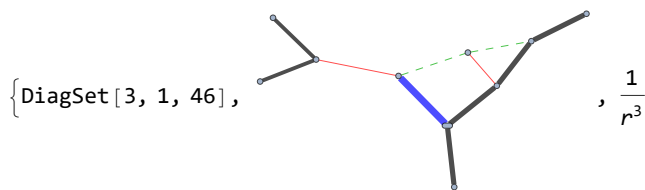
 $\left. , \frac{1}{r^3} \right\}$

$$\begin{aligned}
 & G^3 m_1^2 m_2 \left( \frac{8 \hat{n} \cdot \vec{v}_1 \hat{n} \times \vec{S}_1 \cdot \vec{a}_1 + \frac{8}{3} \vec{S}_1 \times \vec{v}_1 \cdot \vec{a}_1}{\epsilon_d} - 24 \log\left(\frac{r}{R_\theta}\right) \hat{n} \cdot \vec{v}_1 \hat{n} \times \vec{S}_1 \cdot \vec{a}_1 + 8 \hat{n} \cdot \vec{v}_1 \hat{n} \times \vec{S}_1 \cdot \vec{a}_1 - 8 \log\left(\frac{r}{R_\theta}\right) \vec{S}_1 \times \vec{v}_1 \cdot \vec{a}_1 \right) + \\
 & \frac{1}{r^4} G^3 m_1^2 m_2 \left( \frac{1}{\epsilon_d} \left( -16 (\hat{n} \cdot \vec{v}_1)^2 \hat{n} \times \vec{S}_1 \cdot \vec{v}_1 - \frac{16}{5} \hat{n} \cdot \vec{v}_1 \vec{S}_1 \times \vec{v}_1 \cdot \vec{v}_2 + 16 \hat{n} \cdot \vec{v}_2 \hat{n} \cdot \vec{v}_1 \hat{n} \times \vec{S}_1 \cdot \vec{v}_1 + \frac{16}{5} \vec{v}_1 \cdot \vec{v}_1 \hat{n} \times \vec{S}_1 \cdot \vec{v}_1 - \right. \right. \\
 & \left. \frac{16}{5} \vec{v}_1 \cdot \vec{v}_2 \hat{n} \times \vec{S}_1 \cdot \vec{v}_1 \right) + 48 \log\left(\frac{r}{R_\theta}\right) (\hat{n} \cdot \vec{v}_1)^2 \hat{n} \times \vec{S}_1 \cdot \vec{v}_1 + \frac{48}{5} \log\left(\frac{r}{R_\theta}\right) \hat{n} \cdot \vec{v}_1 \vec{S}_1 \times \vec{v}_1 \cdot \vec{v}_2 - 48 \log\left(\frac{r}{R_\theta}\right) \hat{n} \cdot \vec{v}_2 \\
 & \left. \hat{n} \cdot \vec{v}_1 \hat{n} \times \vec{S}_1 \cdot \vec{v}_1 - \frac{48}{5} \log\left(\frac{r}{R_\theta}\right) \vec{v}_1 \cdot \vec{v}_1 \hat{n} \times \vec{S}_1 \cdot \vec{v}_1 + \frac{48}{5} \log\left(\frac{r}{R_\theta}\right) \vec{v}_1 \cdot \vec{v}_2 \hat{n} \times \vec{S}_1 \cdot \vec{v}_1 - 32 (\hat{n} \cdot \vec{v}_1)^2 \hat{n} \times \vec{S}_1 \cdot \vec{v}_1 - \right.
 \end{aligned}$$

$$\frac{112}{25} \hat{n} \cdot \vec{v}_1 \vec{S}_1 \times \vec{v}_1 \cdot \vec{v}_2 + 32 \hat{n} \cdot \vec{v}_2 \hat{n} \cdot \vec{v}_1 \hat{n} \times \vec{S}_1 \cdot \vec{v}_1 + \frac{192}{25} \vec{v}_1 \cdot \vec{v}_1 \hat{n} \times \vec{S}_1 \cdot \vec{v}_1 - \frac{112}{25} \vec{v}_1 \cdot \vec{v}_2 \hat{n} \times \vec{S}_1 \cdot \vec{v}_1 \Big\}$$

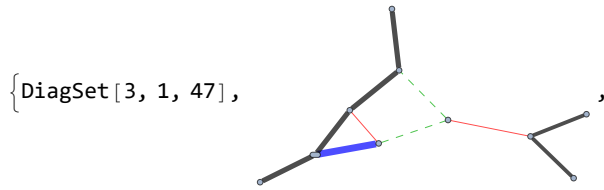

$$\frac{1}{r^3} G^3 m_1^2 m_2 \left( \frac{\frac{4}{5} \hat{n} \cdot \vec{a}_1 \hat{n} \times \vec{S}_1 \cdot \vec{v}_1 - \frac{4}{5} \hat{n} \cdot \vec{v}_1 \hat{n} \times \vec{S}_1 \cdot \vec{a}_1 - \frac{8}{15} \vec{S}_1 \times \vec{v}_1 \cdot \vec{a}_1}{\epsilon_d} - \frac{12}{5} \log\left(\frac{r}{R_\theta}\right) \hat{n} \cdot \vec{a}_1 \hat{n} \times \vec{S}_1 \cdot \vec{v}_1 + \frac{12}{5} \log\left(\frac{r}{R_\theta}\right) \hat{n} \cdot \vec{v}_1 \right. \\ \left. \hat{n} \times \vec{S}_1 \cdot \vec{a}_1 + \frac{58}{25} \hat{n} \cdot \vec{a}_1 \hat{n} \times \vec{S}_1 \cdot \vec{v}_1 - \frac{98}{25} \hat{n} \cdot \vec{v}_1 \hat{n} \times \vec{S}_1 \cdot \vec{a}_1 + \frac{8}{5} \log\left(\frac{r}{R_\theta}\right) \vec{S}_1 \times \vec{v}_1 \cdot \vec{a}_1 - \frac{92}{25} \vec{S}_1 \times \vec{v}_1 \cdot \vec{a}_1 \right) + \frac{1}{r^4} G^3 m_1^2 m_2 \\ \left( 8 (\hat{n} \cdot \vec{v}_1)^2 \hat{n} \times \vec{S}_1 \cdot \vec{v}_1 + \frac{8}{5} \hat{n} \cdot \vec{v}_1 \vec{S}_1 \times \vec{v}_1 \cdot \vec{v}_2 - 8 \hat{n} \cdot \vec{v}_2 \hat{n} \cdot \vec{v}_1 \hat{n} \times \vec{S}_1 \cdot \vec{v}_1 + \frac{4}{5} \vec{v}_1 \cdot \vec{v}_1 \hat{n} \times \vec{S}_1 \cdot \vec{v}_1 + \frac{8}{5} \vec{v}_1 \cdot \vec{v}_2 \hat{n} \times \vec{S}_1 \cdot \vec{v}_1 \right) \Big\}$$

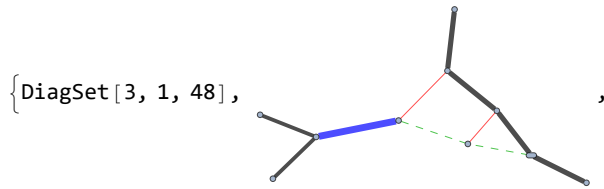

$$\frac{G^3 m_1^2 m_2 \left( -\frac{4 \hat{n} \cdot \vec{v}_2 \hat{n} \times \vec{S}_1 \cdot \vec{v}_2}{5 \epsilon_d} + \frac{12}{5} \log\left(\frac{r}{R_\theta}\right) \hat{n} \cdot \vec{v}_2 \hat{n} \times \vec{S}_1 \cdot \vec{v}_2 - \frac{38}{25} \hat{n} \cdot \vec{v}_2 \hat{n} \times \vec{S}_1 \cdot \vec{v}_2 \right)}{r^3} + \frac{4 G^3 m_1^2 m_2 \hat{n} \cdot \vec{v}_2 \vec{S}_1 \times \vec{v}_1 \cdot \vec{v}_2}{5 r^4} \Big\}$$

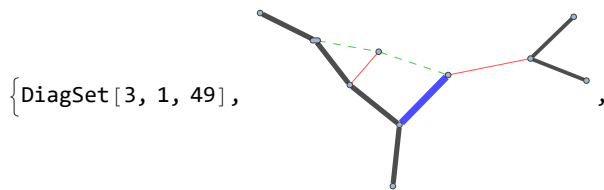

$$\frac{1}{r^4} G^3 m_1^2 m_2 \left( \frac{1}{\epsilon_d} \left( -16 (\hat{n} \cdot \vec{v}_1)^2 \hat{n} \times \vec{S}_1 \cdot \vec{v}_1 - \frac{16}{5} \hat{n} \cdot \vec{v}_1 \vec{S}_1 \times \vec{v}_1 \cdot \vec{v}_2 + 16 \hat{n} \cdot \vec{v}_2 \hat{n} \cdot \vec{v}_1 \hat{n} \times \vec{S}_1 \cdot \vec{v}_1 + \frac{16}{5} \vec{v}_1 \cdot \vec{v}_1 \hat{n} \times \vec{S}_1 \cdot \vec{v}_1 - \right. \right. \\ \left. \frac{16}{5} \vec{v}_1 \cdot \vec{v}_2 \hat{n} \times \vec{S}_1 \cdot \vec{v}_1 \right) + 48 \log\left(\frac{r}{R_\theta}\right) (\hat{n} \cdot \vec{v}_1)^2 \hat{n} \times \vec{S}_1 \cdot \vec{v}_1 + \frac{48}{5} \log\left(\frac{r}{R_\theta}\right) \hat{n} \cdot \vec{v}_1 \vec{S}_1 \times \vec{v}_1 \cdot \vec{v}_2 - 48 \log\left(\frac{r}{R_\theta}\right) \hat{n} \cdot \vec{v}_2 \\ \hat{n} \cdot \vec{v}_1 \hat{n} \times \vec{S}_1 \cdot \vec{v}_1 - \frac{48}{5} \log\left(\frac{r}{R_\theta}\right) \vec{v}_1 \cdot \vec{v}_1 \hat{n} \times \vec{S}_1 \cdot \vec{v}_1 + \frac{48}{5} \log\left(\frac{r}{R_\theta}\right) \vec{v}_1 \cdot \vec{v}_2 \hat{n} \times \vec{S}_1 \cdot \vec{v}_1 - 32 (\hat{n} \cdot \vec{v}_1)^2 \hat{n} \times \vec{S}_1 \cdot \vec{v}_1 - \\ \frac{112}{25} \hat{n} \cdot \vec{v}_1 \vec{S}_1 \times \vec{v}_1 \cdot \vec{v}_2 + 32 \hat{n} \cdot \vec{v}_2 \hat{n} \cdot \vec{v}_1 \hat{n} \times \vec{S}_1 \cdot \vec{v}_1 + \frac{112}{25} \vec{v}_1 \cdot \vec{v}_1 \hat{n} \times \vec{S}_1 \cdot \vec{v}_1 - \frac{112}{25} \vec{v}_1 \cdot \vec{v}_2 \hat{n} \times \vec{S}_1 \cdot \vec{v}_1 \Big) + \\ \frac{G^3 m_1^2 m_2 \left( \frac{4 \hat{n} \cdot \vec{v}_1 \hat{n} \times \vec{S}_1 \cdot \vec{v}_1}{\epsilon_d} - 12 \log\left(\frac{r}{R_\theta}\right) \hat{n} \cdot \vec{v}_1 \hat{n} \times \vec{S}_1 \cdot \vec{v}_1 + 6 \hat{n} \cdot \vec{v}_1 \hat{n} \times \vec{S}_1 \cdot \vec{v}_1 \right)}{r^3} \Big\}$$

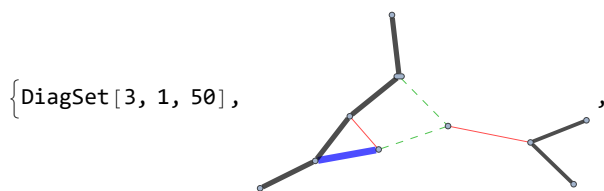

$$\frac{1}{r^4} G^3 m_1^2 m_2 \left( \frac{1}{\epsilon_d} \left( 16 (\hat{n} \cdot \vec{v}_1)^2 \hat{n} \times \vec{S}_1 \cdot \vec{v}_1 + \frac{16}{5} \hat{n} \cdot \vec{v}_1 \vec{S}_1 \times \vec{v}_1 \cdot \vec{v}_2 - 16 \hat{n} \cdot \vec{v}_2 \hat{n} \cdot \vec{v}_1 \hat{n} \times \vec{S}_1 \cdot \vec{v}_1 - \frac{16}{5} \vec{v}_1 \cdot \vec{v}_1 \hat{n} \times \vec{S}_1 \cdot \vec{v}_1 + \right. \right.$$

$$\frac{16}{5} \vec{v}_1 \cdot \vec{v}_2 \hat{n} \times \vec{S}_1 \cdot \vec{v}_1 \Big) - 48 \log \left( \frac{r}{R_\theta} \right) (\hat{n} \cdot \vec{v}_1)^2 \hat{n} \times \vec{S}_1 \cdot \vec{v}_1 - \frac{48}{5} \log \left( \frac{r}{R_\theta} \right) \hat{n} \cdot \vec{v}_1 \vec{S}_1 \times \vec{v}_1 \cdot \vec{v}_2 + 48 \log \left( \frac{r}{R_\theta} \right) \hat{n} \cdot \vec{v}_2 \\ \hat{n} \cdot \vec{v}_1 \hat{n} \times \vec{S}_1 \cdot \vec{v}_1 + \frac{48}{5} \log \left( \frac{r}{R_\theta} \right) \vec{v}_1 \cdot \vec{v}_1 \hat{n} \times \vec{S}_1 \cdot \vec{v}_1 - \frac{48}{5} \log \left( \frac{r}{R_\theta} \right) \vec{v}_1 \cdot \vec{v}_2 \hat{n} \times \vec{S}_1 \cdot \vec{v}_1 + 64 (\hat{n} \cdot \vec{v}_1)^2 \hat{n} \times \vec{S}_1 \cdot \vec{v}_1 + \\ \frac{272}{25} \hat{n} \cdot \vec{v}_1 \vec{S}_1 \times \vec{v}_1 \cdot \vec{v}_2 - 64 \hat{n} \cdot \vec{v}_2 \hat{n} \cdot \vec{v}_1 \hat{n} \times \vec{S}_1 \cdot \vec{v}_1 - \frac{272}{25} \vec{v}_1 \cdot \vec{v}_1 \hat{n} \times \vec{S}_1 \cdot \vec{v}_1 + \frac{272}{25} \vec{v}_1 \cdot \vec{v}_2 \hat{n} \times \vec{S}_1 \cdot \vec{v}_1 \Big) + \\ \frac{G^3 m_1^2 m_2 \left( -\frac{16 \hat{n} \cdot \vec{v}_1 \hat{n} \times \vec{S}_1 \cdot \vec{v}_1}{5 \in_d} + \frac{48}{5} \log \left( \frac{r}{R_\theta} \right) \hat{n} \cdot \vec{v}_1 \hat{n} \times \vec{S}_1 \cdot \vec{v}_1 - \frac{272}{25} \hat{n} \cdot \vec{v}_1 \hat{n} \times \vec{S}_1 \cdot \vec{v}_1 \right)}{r^3} \Big\}$$

$$\left\{ \text{DiagSet}[3, 1, 51], \right. , \frac{1}{r^3}$$
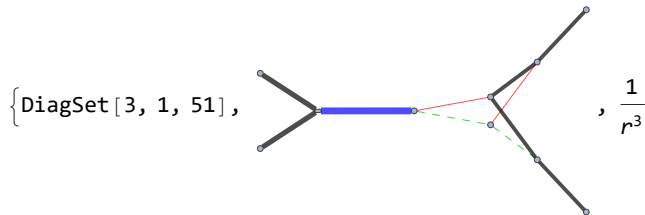

$$G^3 m_2^3 \left( \frac{\frac{8}{3} \vec{a}_2 \times \vec{S}_1 \cdot \vec{v}_1 - 8 \hat{n} \cdot \vec{v}_1 \hat{n} \times \vec{a}_2 \cdot \vec{S}_1}{\in_d} + 24 \log \left( \frac{r}{R_\theta} \right) \hat{n} \cdot \vec{v}_1 \hat{n} \times \vec{a}_2 \cdot \vec{S}_1 - 8 \hat{n} \cdot \vec{v}_1 \hat{n} \times \vec{a}_2 \cdot \vec{S}_1 - 8 \log \left( \frac{r}{R_\theta} \right) \vec{a}_2 \times \vec{S}_1 \cdot \vec{v}_1 \right) \Big\}$$

$$\left\{ \text{DiagSet}[3, 1, 52], \right. ,$$
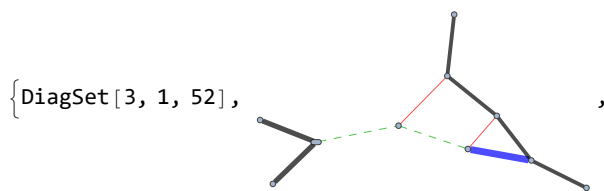

$$\frac{1}{r^4} G^3 m_2^3 \left( -160 (\hat{n} \cdot \vec{v}_2)^2 \hat{n} \times \vec{S}_1 \cdot \vec{v}_2 + 32 \hat{n} \cdot \vec{v}_2 \vec{S}_1 \times \vec{v}_1 \cdot \vec{v}_2 + 160 \hat{n} \cdot \vec{v}_1 \hat{n} \cdot \vec{v}_2 \hat{n} \times \vec{S}_1 \cdot \vec{v}_2 - \right. \\ \left. 32 \vec{v}_1 \cdot \vec{v}_2 \hat{n} \times \vec{S}_1 \cdot \vec{v}_2 + 32 \vec{v}_2 \cdot \vec{v}_2 \hat{n} \times \vec{S}_1 \cdot \vec{v}_2 \right) - \frac{32 G^3 m_2^3 \hat{n} \cdot \vec{v}_2 \hat{n} \times \vec{S}_1 \cdot \vec{v}_2}{r^3} \Big\}$$

$$\left\{ \text{DiagSet}[3, 1, 53], \right. ,$$
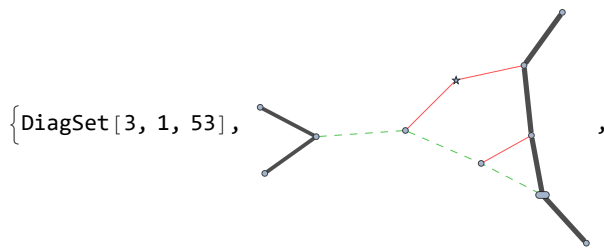

$$\frac{1}{r^3} m_1^2 m_2 \left( \frac{4}{5} \log \left( \frac{r}{R_\theta} \right) \vec{S}_1 \times \vec{v}_1 \cdot \vec{v}_2 - \frac{6}{25} \vec{S}_1 \times \vec{v}_1 \cdot \vec{v}_2 - \frac{6}{25} \vec{S}_1 \times \vec{v}_1 \cdot \vec{a}_2 + \frac{56}{25} \hat{n} \times \vec{S}_1 \cdot \vec{v}_1 \hat{n} \cdot \vec{a}_2 + \frac{98}{25} \hat{n} \times \vec{S}_1 \cdot \vec{v}_2 \hat{n} \cdot \vec{v}_1 + \right. \\ \frac{98}{25} \hat{n} \times \vec{S}_1 \cdot \vec{a}_2 \hat{n} \cdot \vec{v}_1 + \frac{56}{25} \hat{n} \times \vec{S}_1 \cdot \vec{v}_1 \hat{n} \cdot \vec{v}_2 + \frac{4}{5} \vec{S}_1 \times \vec{v}_1 \cdot \vec{a}_2 \log \left( \frac{r}{R_\theta} \right) - \frac{24}{5} \hat{n} \times \vec{S}_1 \cdot \vec{v}_1 \hat{n} \cdot \vec{a}_2 \log \left( \frac{r}{R_\theta} \right) - \\ \frac{12}{5} \hat{n} \times \vec{S}_1 \cdot \vec{v}_2 \hat{n} \cdot \vec{v}_1 \log \left( \frac{r}{R_\theta} \right) - \frac{12}{5} \hat{n} \times \vec{S}_1 \cdot \vec{a}_2 \hat{n} \cdot \vec{v}_1 \log \left( \frac{r}{R_\theta} \right) - \frac{24}{5} \hat{n} \times \vec{S}_1 \cdot \vec{v}_1 \hat{n} \cdot \vec{v}_2 \log \left( \frac{r}{R_\theta} \right) + \frac{1}{\in_d} \left( -\frac{4}{15} \vec{S}_1 \times \vec{v}_1 \cdot \vec{v}_2 - \right. \\ \left. \frac{4}{15} \vec{S}_1 \times \vec{v}_1 \cdot \vec{a}_2 + \frac{8}{5} \hat{n} \times \vec{S}_1 \cdot \vec{v}_1 \hat{n} \cdot \vec{a}_2 + \frac{4}{5} \hat{n} \times \vec{S}_1 \cdot \vec{v}_2 \hat{n} \cdot \vec{v}_1 + \frac{4}{5} \hat{n} \times \vec{S}_1 \cdot \vec{a}_2 \hat{n} \cdot \vec{v}_1 + \frac{8}{5} \hat{n} \times \vec{S}_1 \cdot \vec{v}_1 \hat{n} \cdot \vec{v}_2 \right) \Big) G^3 + \\ \frac{1}{r^4} m_1^2 m_2 \left( -\frac{880}{49} \hat{n} \times \vec{S}_1 \cdot \vec{v}_2 (\hat{n} \cdot \vec{v}_1)^2 + \frac{72}{7} \hat{n} \times \vec{S}_1 \cdot \vec{v}_2 \log \left( \frac{r}{R_\theta} \right) (\hat{n} \cdot \vec{v}_1)^2 - \frac{3912 \vec{S}_1 \times \vec{v}_1 \cdot \vec{v}_2 \hat{n} \cdot \vec{v}_1}{1225} - \right. \\ \left. \frac{496}{49} \hat{n} \times \vec{S}_1 \cdot \vec{v}_1 \hat{n} \cdot \vec{v}_2 \hat{n} \cdot \vec{v}_1 + 22 \hat{n} \times \vec{S}_1 \cdot \vec{v}_2 \hat{n} \cdot \vec{v}_2 \hat{n} \cdot \vec{v}_1 + \frac{24}{35} \vec{S}_1 \times \vec{v}_1 \cdot \vec{v}_2 \log \left( \frac{r}{R_\theta} \right) \hat{n} \cdot \vec{v}_1 + \right.$$

$$\begin{aligned} & \frac{120}{7} \hat{n} \times \vec{S}_1 \cdot \vec{v}_1 \hat{n} \cdot \vec{v}_2 \log\left(\frac{r}{R_\theta}\right) \hat{n} \cdot \vec{v}_1 - 12 \hat{n} \times \vec{S}_1 \cdot \vec{v}_2 \hat{n} \cdot \vec{v}_2 \log\left(\frac{r}{R_\theta}\right) \hat{n} \cdot \vec{v}_1 + 16 \hat{n} \times \vec{S}_1 \cdot \vec{v}_1 (\hat{n} \cdot \vec{v}_2)^2 - \\ & \frac{94}{25} \vec{S}_1 \times \vec{v}_1 \cdot \vec{v}_2 \hat{n} \cdot \vec{v}_2 + \frac{1096 \hat{n} \times \vec{S}_1 \cdot \vec{v}_2 \vec{v}_1 \cdot \vec{v}_1}{1225} + \frac{88}{49} \hat{n} \times \vec{S}_1 \cdot \vec{v}_1 \vec{v}_1 \cdot \vec{v}_2 - \frac{98}{25} \hat{n} \times \vec{S}_1 \cdot \vec{v}_2 \vec{v}_1 \cdot \vec{v}_2 - \\ & \frac{56}{25} \hat{n} \times \vec{S}_1 \cdot \vec{v}_1 \vec{v}_2 \cdot \vec{v}_2 - 24 \hat{n} \times \vec{S}_1 \cdot \vec{v}_1 (\hat{n} \cdot \vec{v}_2)^2 \log\left(\frac{r}{R_\theta}\right) + \frac{36}{5} \vec{S}_1 \times \vec{v}_1 \cdot \vec{v}_2 \hat{n} \cdot \vec{v}_2 \log\left(\frac{r}{R_\theta}\right) - \\ & \frac{72}{35} \hat{n} \times \vec{S}_1 \cdot \vec{v}_2 \vec{v}_1 \cdot \vec{v}_1 \log\left(\frac{r}{R_\theta}\right) - \frac{24}{7} \hat{n} \times \vec{S}_1 \cdot \vec{v}_1 \vec{v}_1 \cdot \vec{v}_2 \log\left(\frac{r}{R_\theta}\right) + \frac{12}{5} \hat{n} \times \vec{S}_1 \cdot \vec{v}_2 \vec{v}_1 \cdot \vec{v}_2 \log\left(\frac{r}{R_\theta}\right) + \\ & \frac{24}{5} \hat{n} \times \vec{S}_1 \cdot \vec{v}_1 \vec{v}_2 \cdot \vec{v}_2 \log\left(\frac{r}{R_\theta}\right) + \frac{1}{\epsilon_d} \left( -\frac{24}{7} \hat{n} \times \vec{S}_1 \cdot \vec{v}_2 (\hat{n} \cdot \vec{v}_1)^2 - \frac{8}{35} \vec{S}_1 \times \vec{v}_1 \cdot \vec{v}_2 \hat{n} \cdot \vec{v}_1 - \right. \\ & \left. \frac{40}{7} \hat{n} \times \vec{S}_1 \cdot \vec{v}_1 \hat{n} \cdot \vec{v}_2 \hat{n} \cdot \vec{v}_1 + 4 \hat{n} \times \vec{S}_1 \cdot \vec{v}_2 \hat{n} \cdot \vec{v}_2 \hat{n} \cdot \vec{v}_1 + 8 \hat{n} \times \vec{S}_1 \cdot \vec{v}_1 (\hat{n} \cdot \vec{v}_2)^2 - \frac{12}{5} \vec{S}_1 \times \vec{v}_1 \cdot \vec{v}_2 \hat{n} \cdot \vec{v}_2 + \right. \\ & \left. \frac{24}{35} \hat{n} \times \vec{S}_1 \cdot \vec{v}_2 \vec{v}_1 \cdot \vec{v}_1 + \frac{8}{7} \hat{n} \times \vec{S}_1 \cdot \vec{v}_1 \vec{v}_1 \cdot \vec{v}_2 - \frac{4}{5} \hat{n} \times \vec{S}_1 \cdot \vec{v}_2 \vec{v}_1 \cdot \vec{v}_2 - \frac{8}{5} \hat{n} \times \vec{S}_1 \cdot \vec{v}_1 \vec{v}_2 \cdot \vec{v}_2 \right) \Bigg\} G^3 \} \end{aligned}$$

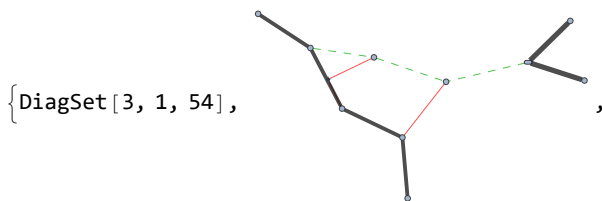

$$\begin{aligned} & \frac{1}{r^3} G^3 m_2^3 \left( \frac{4 \hat{n} \cdot \vec{a}_2 \hat{n} \times \vec{S}_1 \cdot \vec{v}_2 + 4 \hat{n} \cdot \vec{v}_2 \hat{n} \times \vec{a}_2 \cdot \vec{S}_1 - \frac{8}{3} \vec{a}_2 \times \vec{S}_1 \cdot \vec{v}_2}{\epsilon_d} - 12 \log\left(\frac{r}{R_\theta}\right) \hat{n} \cdot \vec{a}_2 \hat{n} \times \vec{S}_1 \cdot \vec{v}_2 - 12 \log\left(\frac{r}{R_\theta}\right) \hat{n} \cdot \vec{v}_2 \right. \\ & \left. \hat{n} \times \vec{a}_2 \cdot \vec{S}_1 - 4 \hat{n} \cdot \vec{a}_2 \hat{n} \times \vec{S}_1 \cdot \vec{v}_2 + 12 \hat{n} \cdot \vec{v}_2 \hat{n} \times \vec{a}_2 \cdot \vec{S}_1 + 8 \log\left(\frac{r}{R_\theta}\right) \vec{a}_2 \times \vec{S}_1 \cdot \vec{v}_2 - 16 \hat{n} \cdot \vec{v}_2 \hat{n} \times \vec{S}_1 \cdot \vec{v}_2 \right) + \frac{1}{r^4} \\ & G^3 m_2^3 \left( -64 (\hat{n} \cdot \vec{v}_2)^2 \hat{n} \times \vec{S}_1 \cdot \vec{v}_2 + 16 \hat{n} \cdot \vec{v}_2 \vec{S}_1 \times \vec{v}_1 \cdot \vec{v}_2 + 80 \hat{n} \cdot \vec{v}_1 \hat{n} \cdot \vec{v}_2 \hat{n} \times \vec{S}_1 \cdot \vec{v}_2 - 16 \vec{v}_1 \cdot \vec{v}_2 \hat{n} \times \vec{S}_1 \cdot \vec{v}_2 \right) \Bigg\} \end{aligned}$$

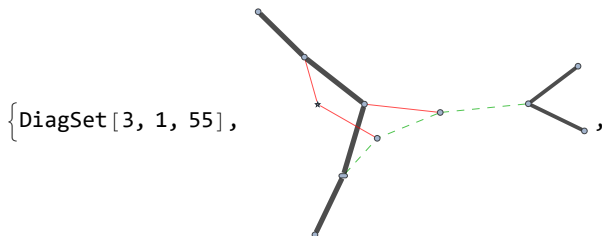

$$\begin{aligned} & \frac{1}{r^3} m_1^2 m_2 \left( \frac{38}{5} \log\left(\frac{r}{R_\theta}\right) \vec{S}_1 \times \vec{v}_1 \cdot \vec{v}_2 - \frac{91}{75} \vec{S}_1 \times \vec{v}_1 \cdot \vec{v}_2 - \frac{91}{75} \vec{S}_1 \times \vec{v}_1 \cdot \vec{a}_2 + \frac{97}{25} \hat{n} \times \vec{S}_1 \cdot \vec{v}_1 \hat{n} \cdot \vec{a}_2 + \frac{76}{25} \hat{n} \times \vec{S}_1 \cdot \vec{v}_2 \hat{n} \cdot \vec{v}_1 + \right. \\ & \frac{76}{25} \hat{n} \times \vec{S}_1 \cdot \vec{a}_2 \hat{n} \cdot \vec{v}_1 + \frac{97}{25} \hat{n} \times \vec{S}_1 \cdot \vec{v}_1 \hat{n} \cdot \vec{v}_2 + \frac{38}{5} \vec{S}_1 \times \vec{v}_1 \cdot \vec{a}_2 \log\left(\frac{r}{R_\theta}\right) - \frac{78}{5} \hat{n} \times \vec{S}_1 \cdot \vec{v}_1 \hat{n} \cdot \vec{a}_2 \log\left(\frac{r}{R_\theta}\right) + \\ & \frac{36}{5} \hat{n} \times \vec{S}_1 \cdot \vec{v}_2 \hat{n} \cdot \vec{v}_1 \log\left(\frac{r}{R_\theta}\right) + \frac{36}{5} \hat{n} \times \vec{S}_1 \cdot \vec{a}_2 \hat{n} \cdot \vec{v}_1 \log\left(\frac{r}{R_\theta}\right) - \frac{78}{5} \hat{n} \times \vec{S}_1 \cdot \vec{v}_1 \hat{n} \cdot \vec{v}_2 \log\left(\frac{r}{R_\theta}\right) + \frac{1}{\epsilon_d} \left( -\frac{38}{15} \vec{S}_1 \times \vec{v}_1 \cdot \vec{v}_2 - \right. \\ & \left. \frac{38}{15} \vec{S}_1 \times \vec{v}_1 \cdot \vec{a}_2 + \frac{26}{5} \hat{n} \times \vec{S}_1 \cdot \vec{v}_1 \hat{n} \cdot \vec{a}_2 - \frac{12}{5} \hat{n} \times \vec{S}_1 \cdot \vec{v}_2 \hat{n} \cdot \vec{v}_1 - \frac{12}{5} \hat{n} \times \vec{S}_1 \cdot \vec{a}_2 \hat{n} \cdot \vec{v}_1 + \frac{26}{5} \hat{n} \times \vec{S}_1 \cdot \vec{v}_1 \hat{n} \cdot \vec{v}_2 \right) \Bigg\} G^3 + \\ & \frac{1}{r^4} m_1^2 m_2 \left( -\frac{344}{49} \hat{n} \times \vec{S}_1 \cdot \vec{v}_2 (\hat{n} \cdot \vec{v}_1)^2 - \frac{204}{7} \hat{n} \times \vec{S}_1 \cdot \vec{v}_2 \log\left(\frac{r}{R_\theta}\right) (\hat{n} \cdot \vec{v}_1)^2 + \frac{597}{245} \vec{S}_1 \times \vec{v}_1 \cdot \vec{v}_2 \hat{n} \cdot \vec{v}_1 - \right. \\ & \frac{1075}{49} \hat{n} \times \vec{S}_1 \cdot \vec{v}_1 \hat{n} \cdot \vec{v}_2 \hat{n} \cdot \vec{v}_1 + 8 \hat{n} \times \vec{S}_1 \cdot \vec{v}_2 \hat{n} \cdot \vec{v}_2 \hat{n} \cdot \vec{v}_1 - \frac{162}{7} \vec{S}_1 \times \vec{v}_1 \cdot \vec{v}_2 \log\left(\frac{r}{R_\theta}\right) \hat{n} \cdot \vec{v}_1 + \\ & \left. \frac{402}{7} \hat{n} \times \vec{S}_1 \cdot \vec{v}_1 \hat{n} \cdot \vec{v}_2 \log\left(\frac{r}{R_\theta}\right) \hat{n} \cdot \vec{v}_1 + 36 \hat{n} \times \vec{S}_1 \cdot \vec{v}_2 \hat{n} \cdot \vec{v}_2 \log\left(\frac{r}{R_\theta}\right) \hat{n} \cdot \vec{v}_1 + 35 \hat{n} \times \vec{S}_1 \cdot \vec{v}_1 (\hat{n} \cdot \vec{v}_2)^2 - \right. \end{aligned}$$

$$\begin{aligned}
& \frac{378}{25} \vec{S}_1 \times \vec{v}_1 \cdot \vec{v}_2 \hat{n} \cdot \vec{v}_2 - \frac{1332 \hat{n} \times \vec{S}_1 \cdot \vec{v}_2 \vec{v}_1 \cdot \vec{v}_1}{1225} + \frac{5221 \hat{n} \times \vec{S}_1 \cdot \vec{v}_1 \vec{v}_1 \cdot \vec{v}_2}{1225} - \frac{76}{25} \hat{n} \times \vec{S}_1 \cdot \vec{v}_2 \vec{v}_1 \cdot \vec{v}_2 - \\
& \frac{97}{25} \hat{n} \times \vec{S}_1 \cdot \vec{v}_1 \vec{v}_2 \cdot \vec{v}_2 - 78 \hat{n} \times \vec{S}_1 \cdot \vec{v}_1 (\hat{n} \cdot \vec{v}_2)^2 \log\left(\frac{r}{R_\theta}\right) + \frac{192}{5} \vec{S}_1 \times \vec{v}_1 \cdot \vec{v}_2 \hat{n} \cdot \vec{v}_2 \log\left(\frac{r}{R_\theta}\right) + \\
& \frac{204}{35} \hat{n} \times \vec{S}_1 \cdot \vec{v}_2 \vec{v}_1 \cdot \vec{v}_1 \log\left(\frac{r}{R_\theta}\right) - \frac{402}{35} \hat{n} \times \vec{S}_1 \cdot \vec{v}_1 \vec{v}_1 \cdot \vec{v}_2 \log\left(\frac{r}{R_\theta}\right) - \frac{36}{5} \hat{n} \times \vec{S}_1 \cdot \vec{v}_2 \vec{v}_1 \cdot \vec{v}_2 \log\left(\frac{r}{R_\theta}\right) + \\
& \frac{78}{5} \hat{n} \times \vec{S}_1 \cdot \vec{v}_1 \vec{v}_2 \cdot \vec{v}_2 \log\left(\frac{r}{R_\theta}\right) + \frac{1}{\epsilon_d} \left( \frac{68}{7} \hat{n} \times \vec{S}_1 \cdot \vec{v}_2 (\hat{n} \cdot \vec{v}_1)^2 + \frac{54}{7} \vec{S}_1 \times \vec{v}_1 \cdot \vec{v}_2 \hat{n} \cdot \vec{v}_1 - \right. \\
& \left. \frac{134}{7} \hat{n} \times \vec{S}_1 \cdot \vec{v}_1 \hat{n} \cdot \vec{v}_2 \hat{n} \cdot \vec{v}_1 - 12 \hat{n} \times \vec{S}_1 \cdot \vec{v}_2 \hat{n} \cdot \vec{v}_2 \hat{n} \cdot \vec{v}_1 + 26 \hat{n} \times \vec{S}_1 \cdot \vec{v}_1 (\hat{n} \cdot \vec{v}_2)^2 - \frac{64}{5} \vec{S}_1 \times \vec{v}_1 \cdot \vec{v}_2 \hat{n} \cdot \vec{v}_2 - \right. \\
& \left. \frac{68}{35} \hat{n} \times \vec{S}_1 \cdot \vec{v}_2 \vec{v}_1 \cdot \vec{v}_1 + \frac{134}{35} \hat{n} \times \vec{S}_1 \cdot \vec{v}_1 \vec{v}_1 \cdot \vec{v}_2 + \frac{12}{5} \hat{n} \times \vec{S}_1 \cdot \vec{v}_2 \vec{v}_1 \cdot \vec{v}_2 - \frac{26}{5} \hat{n} \times \vec{S}_1 \cdot \vec{v}_1 \vec{v}_2 \cdot \vec{v}_2 \right) \Bigg\} G^3 \Bigg\}
\end{aligned}$$

$\{\text{DiagSet}[3, 1, 56],$ 
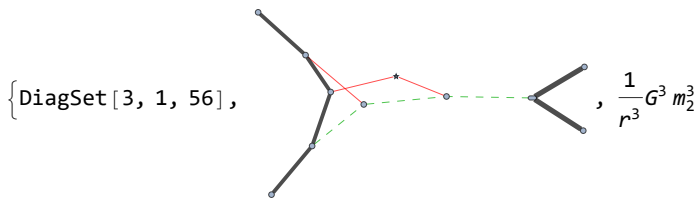
 $, \frac{1}{r^3} G^3 m_2^3$

$$\begin{aligned}
& \left( \frac{8 \hat{n} \cdot \vec{a}_2 \hat{n} \times \vec{S}_1 \cdot \vec{v}_2 + 8 \hat{n} \cdot \vec{v}_2 \hat{n} \times \vec{a}_2 \cdot \vec{S}_1 - \frac{16}{3} \vec{a}_2 \times \vec{S}_1 \cdot \vec{v}_2}{\epsilon_d} - 24 \log\left(\frac{r}{R_\theta}\right) \hat{n} \cdot \vec{a}_2 \hat{n} \times \vec{S}_1 \cdot \vec{v}_2 - 24 \log\left(\frac{r}{R_\theta}\right) \hat{n} \cdot \vec{v}_2 \hat{n} \times \vec{a}_2 \cdot \vec{S}_1 + \right. \\
& \left. 8 \hat{n} \cdot \vec{a}_2 \hat{n} \times \vec{S}_1 \cdot \vec{v}_2 + 24 \hat{n} \cdot \vec{v}_2 \hat{n} \times \vec{a}_2 \cdot \vec{S}_1 + 16 \log\left(\frac{r}{R_\theta}\right) \vec{a}_2 \times \vec{S}_1 \cdot \vec{v}_2 - \frac{16}{3} \vec{a}_2 \times \vec{S}_1 \cdot \vec{v}_2 - 16 \hat{n} \cdot \vec{v}_2 \hat{n} \times \vec{S}_1 \cdot \vec{v}_2 \right) + \\
& \frac{1}{r^4} G^3 m_2^3 \left( -64 (\hat{n} \cdot \vec{v}_2)^2 \hat{n} \times \vec{S}_1 \cdot \vec{v}_2 + 16 \hat{n} \cdot \vec{v}_2 \vec{S}_1 \times \vec{v}_1 \cdot \vec{v}_2 + 80 \hat{n} \cdot \vec{v}_1 \hat{n} \cdot \vec{v}_2 \hat{n} \times \vec{S}_1 \cdot \vec{v}_2 - 16 \vec{v}_1 \cdot \vec{v}_2 \hat{n} \times \vec{S}_1 \cdot \vec{v}_2 \right) \Bigg\}
\end{aligned}$$

$\{\text{DiagSet}[3, 1, 57],$ 
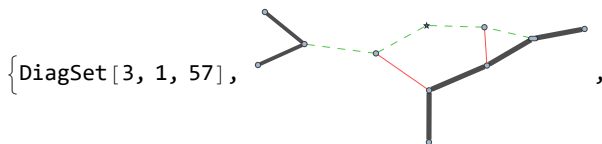
 $,$

$$\begin{aligned}
& \frac{m_1^2 m_2 \left( -4 \log\left(\frac{r}{R_\theta}\right) \hat{n} \times \vec{S}_1 \cdot \vec{a}_2 + \frac{4 \hat{n} \times \vec{S}_1 \cdot \vec{a}_2}{3 \epsilon_d} - \frac{2}{3} \hat{n} \times \vec{S}_1 \cdot \vec{a}_2 \right) G^3}{r^2} + \frac{1}{r^3} m_1^2 m_2 \\
& \left( \frac{12}{5} \log\left(\frac{r}{R_\theta}\right) \vec{S}_1 \times \vec{v}_1 \cdot \vec{v}_2 - \frac{74}{75} \vec{S}_1 \times \vec{v}_1 \cdot \vec{v}_2 + \frac{124}{75} \vec{S}_1 \times \vec{v}_1 \cdot \vec{a}_2 - \frac{58}{25} \hat{n} \times \vec{S}_1 \cdot \vec{v}_1 \hat{n} \cdot \vec{a}_2 - \frac{36}{25} \hat{n} \times \vec{S}_1 \cdot \vec{v}_2 \hat{n} \cdot \vec{v}_1 - \frac{14}{25} \hat{n} \times \vec{S}_1 \cdot \vec{a}_2 \right. \\
& \left. \hat{n} \cdot \vec{v}_1 + \frac{58}{25} \hat{n} \times \vec{S}_1 \cdot \vec{v}_1 \hat{n} \cdot \vec{v}_2 + 2 \hat{n} \times \vec{S}_1 \cdot \vec{v}_2 \hat{n} \cdot \vec{v}_2 + \frac{8}{5} \vec{S}_1 \times \vec{v}_1 \cdot \vec{a}_2 \log\left(\frac{r}{R_\theta}\right) + \frac{12}{5} \hat{n} \times \vec{S}_1 \cdot \vec{v}_1 \hat{n} \cdot \vec{a}_2 \log\left(\frac{r}{R_\theta}\right) + \right. \\
& \left. \frac{24}{5} \hat{n} \times \vec{S}_1 \cdot \vec{v}_2 \hat{n} \cdot \vec{v}_1 \log\left(\frac{r}{R_\theta}\right) + \frac{36}{5} \hat{n} \times \vec{S}_1 \cdot \vec{a}_2 \hat{n} \cdot \vec{v}_1 \log\left(\frac{r}{R_\theta}\right) - \frac{12}{5} \hat{n} \times \vec{S}_1 \cdot \vec{v}_1 \hat{n} \cdot \vec{v}_2 \log\left(\frac{r}{R_\theta}\right) - \right. \\
& \left. 12 \hat{n} \times \vec{S}_1 \cdot \vec{v}_2 \hat{n} \cdot \vec{v}_2 \log\left(\frac{r}{R_\theta}\right) + \frac{1}{\epsilon_d} \left( -\frac{4}{5} \vec{S}_1 \times \vec{v}_1 \cdot \vec{v}_2 - \frac{8}{15} \vec{S}_1 \times \vec{v}_1 \cdot \vec{a}_2 - \frac{4}{5} \hat{n} \times \vec{S}_1 \cdot \vec{v}_1 \hat{n} \cdot \vec{a}_2 - \right. \right. \\
& \left. \left. \frac{8}{5} \hat{n} \times \vec{S}_1 \cdot \vec{v}_2 \hat{n} \cdot \vec{v}_1 - \frac{12}{5} \hat{n} \times \vec{S}_1 \cdot \vec{a}_2 \hat{n} \cdot \vec{v}_1 + \frac{4}{5} \hat{n} \times \vec{S}_1 \cdot \vec{v}_1 \hat{n} \cdot \vec{v}_2 + 4 \hat{n} \times \vec{S}_1 \cdot \vec{v}_2 \hat{n} \cdot \vec{v}_2 \right) \right) \Bigg\} G^3 + \\
& \frac{1}{r^4} m_1^2 m_2 \left( \frac{234}{49} \hat{n} \times \vec{S}_1 \cdot \vec{v}_2 (\hat{n} \cdot \vec{v}_1)^2 - \frac{60}{7} \hat{n} \times \vec{S}_1 \cdot \vec{v}_2 \log\left(\frac{r}{R_\theta}\right) (\hat{n} \cdot \vec{v}_1)^2 + \frac{1426 \vec{S}_1 \times \vec{v}_1 \cdot \vec{v}_2 \hat{n} \cdot \vec{v}_1}{1225} - \right. \\
& \left. \frac{114}{49} \hat{n} \times \vec{S}_1 \cdot \vec{v}_1 \hat{n} \cdot \vec{v}_2 \hat{n} \cdot \vec{v}_1 - 10 \hat{n} \times \vec{S}_1 \cdot \vec{v}_2 \hat{n} \cdot \vec{v}_2 \hat{n} \cdot \vec{v}_1 - \frac{132}{35} \vec{S}_1 \times \vec{v}_1 \cdot \vec{v}_2 \log\left(\frac{r}{R_\theta}\right) \hat{n} \cdot \vec{v}_1 + \right.
\end{aligned}$$



$$\begin{aligned} & \frac{12}{7} \hat{n} \times \vec{S}_1 \cdot \vec{v}_1 \hat{n} \cdot \vec{v}_2 \log\left(\frac{r}{R_\theta}\right) \hat{n} \cdot \vec{v}_1 + 36 \hat{n} \times \vec{S}_1 \cdot \vec{v}_2 \hat{n} \cdot \vec{v}_2 \log\left(\frac{r}{R_\theta}\right) \hat{n} \cdot \vec{v}_1 - 14 \hat{n} \times \vec{S}_1 \cdot \vec{v}_1 (\hat{n} \cdot \vec{v}_2)^2 + \\ & \frac{142}{25} \vec{S}_1 \times \vec{v}_1 \cdot \vec{v}_2 \hat{n} \cdot \vec{v}_2 - \frac{206}{245} \hat{n} \times \vec{S}_1 \cdot \vec{v}_2 \vec{v}_1 \cdot \vec{v}_1 + \frac{1326 \hat{n} \times \vec{S}_1 \cdot \vec{v}_1 \vec{v}_1 \cdot \vec{v}_2}{1225} + \frac{14}{25} \hat{n} \times \vec{S}_1 \cdot \vec{v}_2 \vec{v}_1 \cdot \vec{v}_2 + \\ & \frac{58}{25} \hat{n} \times \vec{S}_1 \cdot \vec{v}_1 \vec{v}_2 \cdot \vec{v}_2 + 12 \hat{n} \times \vec{S}_1 \cdot \vec{v}_1 (\hat{n} \cdot \vec{v}_2)^2 \log\left(\frac{r}{R_\theta}\right) + \frac{12}{5} \vec{S}_1 \times \vec{v}_1 \cdot \vec{v}_2 \hat{n} \cdot \vec{v}_2 \log\left(\frac{r}{R_\theta}\right) + \\ & \frac{12}{7} \hat{n} \times \vec{S}_1 \cdot \vec{v}_2 \vec{v}_1 \cdot \vec{v}_1 \log\left(\frac{r}{R_\theta}\right) - \frac{12}{35} \hat{n} \times \vec{S}_1 \cdot \vec{v}_1 \vec{v}_1 \cdot \vec{v}_2 \log\left(\frac{r}{R_\theta}\right) - \frac{36}{5} \hat{n} \times \vec{S}_1 \cdot \vec{v}_2 \vec{v}_1 \cdot \vec{v}_2 \log\left(\frac{r}{R_\theta}\right) - \\ & \frac{12}{5} \hat{n} \times \vec{S}_1 \cdot \vec{v}_1 \vec{v}_2 \cdot \vec{v}_2 \log\left(\frac{r}{R_\theta}\right) + \frac{1}{\epsilon_d} \left( \frac{20}{7} \hat{n} \times \vec{S}_1 \cdot \vec{v}_2 (\hat{n} \cdot \vec{v}_1)^2 + \frac{44}{35} \vec{S}_1 \times \vec{v}_1 \cdot \vec{v}_2 \hat{n} \cdot \vec{v}_1 - \right. \\ & \left. \frac{4}{7} \hat{n} \times \vec{S}_1 \cdot \vec{v}_1 \hat{n} \cdot \vec{v}_2 \hat{n} \cdot \vec{v}_1 - 12 \hat{n} \times \vec{S}_1 \cdot \vec{v}_2 \hat{n} \cdot \vec{v}_2 \hat{n} \cdot \vec{v}_1 - 4 \hat{n} \times \vec{S}_1 \cdot \vec{v}_1 (\hat{n} \cdot \vec{v}_2)^2 - \frac{4}{5} \vec{S}_1 \times \vec{v}_1 \cdot \vec{v}_2 \hat{n} \cdot \vec{v}_2 - \right. \\ & \left. \frac{4}{7} \hat{n} \times \vec{S}_1 \cdot \vec{v}_2 \vec{v}_1 \cdot \vec{v}_1 + \frac{4}{35} \hat{n} \times \vec{S}_1 \cdot \vec{v}_1 \vec{v}_1 \cdot \vec{v}_2 + \frac{12}{5} \hat{n} \times \vec{S}_1 \cdot \vec{v}_2 \vec{v}_1 \cdot \vec{v}_2 + \frac{4}{5} \hat{n} \times \vec{S}_1 \cdot \vec{v}_1 \vec{v}_2 \cdot \vec{v}_2 \right) \Bigg\} \end{aligned}$$

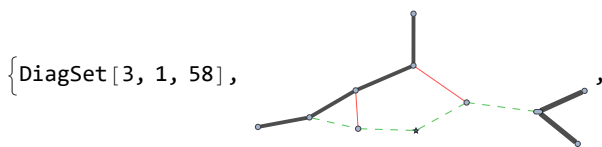

$$\begin{aligned} & \frac{1}{r^3} G^3 m_2^3 \left( \frac{8 \hat{n} \cdot \vec{a}_2 \hat{n} \times \vec{S}_1 \cdot \vec{v}_2 + 8 \hat{n} \cdot \vec{v}_2 \hat{n} \times \vec{a}_2 \cdot \vec{S}_1 - \frac{16}{3} \vec{a}_2 \times \vec{S}_1 \cdot \vec{v}_2}{\epsilon_d} - 24 \log\left(\frac{r}{R_\theta}\right) \hat{n} \cdot \vec{a}_2 \hat{n} \times \vec{S}_1 \cdot \vec{v}_2 - \right. \\ & 24 \log\left(\frac{r}{R_\theta}\right) \hat{n} \cdot \vec{v}_2 \hat{n} \times \vec{a}_2 \cdot \vec{S}_1 + 16 \hat{n} \cdot \vec{a}_2 \hat{n} \times \vec{S}_1 \cdot \vec{v}_2 - 48 \hat{n} \cdot \vec{v}_1 \hat{n} \times \vec{a}_2 \cdot \vec{S}_1 + 32 \hat{n} \cdot \vec{v}_2 \hat{n} \times \vec{a}_2 \cdot \vec{S}_1 + \\ & 16 \log\left(\frac{r}{R_\theta}\right) \vec{a}_2 \times \vec{S}_1 \cdot \vec{v}_2 + 16 \vec{a}_2 \times \vec{S}_1 \cdot \vec{v}_1 - \frac{32}{3} \vec{a}_2 \times \vec{S}_1 \cdot \vec{v}_2 - 32 \hat{n} \cdot \vec{v}_2 \hat{n} \times \vec{S}_1 \cdot \vec{v}_2 \Bigg) + \frac{16 G^3 m_2^3 \hat{n} \times \vec{a}_2 \cdot \vec{S}_1}{r^2} + \frac{1}{r^4} \\ & G^3 m_2^3 \left( -32 (\hat{n} \cdot \vec{v}_2)^2 \hat{n} \times \vec{S}_1 \cdot \vec{v}_2 + 32 \hat{n} \cdot \vec{v}_2 \vec{S}_1 \times \vec{v}_1 \cdot \vec{v}_2 + 160 \hat{n} \cdot \vec{v}_1 \hat{n} \cdot \vec{v}_2 \hat{n} \times \vec{S}_1 \cdot \vec{v}_2 - 32 \vec{v}_1 \cdot \vec{v}_2 \hat{n} \times \vec{S}_1 \cdot \vec{v}_2 \right) \Bigg\} \end{aligned}$$

{DiagSet[3, 1, 59],

$$, \frac{m_1^2 m_2 \left( -24 \log\left(\frac{r}{R_\theta}\right) \hat{n} \times \vec{S}_1 \cdot \vec{a}_2 + \frac{8 \hat{n} \times \vec{S}_1 \cdot \vec{a}_2}{\epsilon_d} - \frac{32}{3} \hat{n} \times \vec{S}_1 \cdot \vec{a}_2 \right) G^3}{r^2} +$$

$$\begin{aligned} & \frac{1}{r^3} m_1^2 m_2 \left( \frac{106}{5} \log\left(\frac{r}{R_\theta}\right) \vec{S}_1 \times \vec{v}_1 \cdot \vec{v}_2 + \frac{203}{75} \vec{S}_1 \times \vec{v}_1 \cdot \vec{v}_2 + \frac{199}{25} \vec{S}_1 \times \vec{v}_1 \cdot \vec{a}_2 - \frac{199}{25} \hat{n} \times \vec{S}_1 \cdot \vec{v}_1 \hat{n} \cdot \vec{a}_2 + \frac{92}{25} \hat{n} \times \vec{S}_1 \cdot \vec{v}_2 \hat{n} \cdot \vec{v}_1 + \right. \\ & \frac{108}{25} \hat{n} \times \vec{S}_1 \cdot \vec{a}_2 \hat{n} \cdot \vec{v}_1 + \frac{199}{25} \hat{n} \times \vec{S}_1 \cdot \vec{v}_1 \hat{n} \cdot \vec{v}_2 - 8 \hat{n} \times \vec{S}_1 \cdot \vec{v}_2 \hat{n} \cdot \vec{v}_2 + \frac{14}{5} \vec{S}_1 \times \vec{v}_1 \cdot \vec{a}_2 \log\left(\frac{r}{R_\theta}\right) + \\ & \frac{66}{5} \hat{n} \times \vec{S}_1 \cdot \vec{v}_1 \hat{n} \cdot \vec{a}_2 \log\left(\frac{r}{R_\theta}\right) + \frac{252}{5} \hat{n} \times \vec{S}_1 \cdot \vec{v}_2 \hat{n} \cdot \vec{v}_1 \log\left(\frac{r}{R_\theta}\right) + \frac{108}{5} \hat{n} \times \vec{S}_1 \cdot \vec{a}_2 \hat{n} \cdot \vec{v}_1 \log\left(\frac{r}{R_\theta}\right) - \\ & \frac{66}{5} \hat{n} \times \vec{S}_1 \cdot \vec{v}_1 \hat{n} \cdot \vec{v}_2 \log\left(\frac{r}{R_\theta}\right) - 72 \hat{n} \times \vec{S}_1 \cdot \vec{v}_2 \hat{n} \cdot \vec{v}_2 \log\left(\frac{r}{R_\theta}\right) + \frac{1}{\epsilon_d} \left( -\frac{106}{15} \vec{S}_1 \times \vec{v}_1 \cdot \vec{v}_2 - \frac{14}{15} \vec{S}_1 \times \vec{v}_1 \cdot \vec{a}_2 - \right. \\ & \left. \frac{22}{5} \hat{n} \times \vec{S}_1 \cdot \vec{v}_1 \hat{n} \cdot \vec{a}_2 - \frac{84}{5} \hat{n} \times \vec{S}_1 \cdot \vec{v}_2 \hat{n} \cdot \vec{v}_1 - \frac{36}{5} \hat{n} \times \vec{S}_1 \cdot \vec{a}_2 \hat{n} \cdot \vec{v}_1 + \frac{22}{5} \hat{n} \times \vec{S}_1 \cdot \vec{v}_1 \hat{n} \cdot \vec{v}_2 + 24 \hat{n} \times \vec{S}_1 \cdot \vec{v}_2 \hat{n} \cdot \vec{v}_2 \right) \Bigg) G^3 + \\ & \frac{1}{r^4} m_1^2 m_2 \left( \frac{432}{49} \hat{n} \times \vec{S}_1 \cdot \vec{v}_2 (\hat{n} \cdot \vec{v}_1)^2 - \frac{324}{7} \hat{n} \times \vec{S}_1 \cdot \vec{v}_2 \log\left(\frac{r}{R_\theta}\right) (\hat{n} \cdot \vec{v}_1)^2 - \frac{1879}{245} \vec{S}_1 \times \vec{v}_1 \cdot \vec{v}_2 \hat{n} \cdot \vec{v}_1 + \right. \\ & \frac{517}{49} \hat{n} \times \vec{S}_1 \cdot \vec{v}_1 \hat{n} \cdot \vec{v}_2 \hat{n} \cdot \vec{v}_1 - \frac{114}{7} \vec{S}_1 \times \vec{v}_1 \cdot \vec{v}_2 \log\left(\frac{r}{R_\theta}\right) \hat{n} \cdot \vec{v}_1 - \frac{78}{7} \hat{n} \times \vec{S}_1 \cdot \vec{v}_1 \hat{n} \cdot \vec{v}_2 \log\left(\frac{r}{R_\theta}\right) \hat{n} \cdot \vec{v}_1 + \\ & 108 \hat{n} \times \vec{S}_1 \cdot \vec{v}_2 \hat{n} \cdot \vec{v}_2 \log\left(\frac{r}{R_\theta}\right) \hat{n} \cdot \vec{v}_1 - 53 \hat{n} \times \vec{S}_1 \cdot \vec{v}_1 (\hat{n} \cdot \vec{v}_2)^2 + \frac{726}{25} \vec{S}_1 \times \vec{v}_1 \cdot \vec{v}_2 \hat{n} \cdot \vec{v}_2 + \end{aligned}$$

$$\begin{aligned}
& \frac{948 \hat{n} \times \vec{S}_1 \cdot \vec{v}_2 \vec{v}_1 \cdot \vec{v}_1}{1225} + \frac{3281 \hat{n} \times \vec{S}_1 \cdot \vec{v}_1 \vec{v}_1 \cdot \vec{v}_2}{1225} - \frac{108}{25} \hat{n} \times \vec{S}_1 \cdot \vec{v}_2 \vec{v}_1 \cdot \vec{v}_2 + \\
& \frac{199}{25} \hat{n} \times \vec{S}_1 \cdot \vec{v}_1 \vec{v}_2 \cdot \vec{v}_2 + 66 \hat{n} \times \vec{S}_1 \cdot \vec{v}_1 (\hat{n} \cdot \vec{v}_2)^2 \log\left(\frac{r}{R_\theta}\right) - \frac{24}{5} \vec{S}_1 \times \vec{v}_1 \cdot \vec{v}_2 \hat{n} \cdot \vec{v}_2 \log\left(\frac{r}{R_\theta}\right) + \\
& \frac{324}{35} \hat{n} \times \vec{S}_1 \cdot \vec{v}_2 \vec{v}_1 \cdot \vec{v}_1 \log\left(\frac{r}{R_\theta}\right) + \frac{78}{35} \hat{n} \times \vec{S}_1 \cdot \vec{v}_1 \vec{v}_1 \cdot \vec{v}_2 \log\left(\frac{r}{R_\theta}\right) - \frac{108}{5} \hat{n} \times \vec{S}_1 \cdot \vec{v}_2 \vec{v}_1 \cdot \vec{v}_2 \log\left(\frac{r}{R_\theta}\right) - \\
& \frac{66}{5} \hat{n} \times \vec{S}_1 \cdot \vec{v}_1 \vec{v}_2 \cdot \vec{v}_2 \log\left(\frac{r}{R_\theta}\right) + \frac{1}{\epsilon_d} \left( \frac{108}{7} \hat{n} \times \vec{S}_1 \cdot \vec{v}_2 (\hat{n} \cdot \vec{v}_1)^2 + \frac{38}{7} \vec{S}_1 \times \vec{v}_1 \cdot \vec{v}_2 \hat{n} \cdot \vec{v}_1 + \right. \\
& \left. \frac{26}{7} \hat{n} \times \vec{S}_1 \cdot \vec{v}_1 \hat{n} \cdot \vec{v}_2 \hat{n} \cdot \vec{v}_1 - 36 \hat{n} \times \vec{S}_1 \cdot \vec{v}_2 \hat{n} \cdot \vec{v}_2 \hat{n} \cdot \vec{v}_1 - 22 \hat{n} \times \vec{S}_1 \cdot \vec{v}_1 (\hat{n} \cdot \vec{v}_2)^2 + \frac{8}{5} \vec{S}_1 \times \vec{v}_1 \cdot \vec{v}_2 \hat{n} \cdot \vec{v}_2 - \right. \\
& \left. \frac{108}{35} \hat{n} \times \vec{S}_1 \cdot \vec{v}_2 \vec{v}_1 \cdot \vec{v}_1 - \frac{26}{35} \hat{n} \times \vec{S}_1 \cdot \vec{v}_1 \vec{v}_1 \cdot \vec{v}_2 + \frac{36}{5} \hat{n} \times \vec{S}_1 \cdot \vec{v}_2 \vec{v}_1 \cdot \vec{v}_2 + \frac{22}{5} \hat{n} \times \vec{S}_1 \cdot \vec{v}_1 \vec{v}_2 \cdot \vec{v}_2 \right) \Bigg\} G^3 \Bigg\}
\end{aligned}$$

{DiagSet[3, 1, 60],

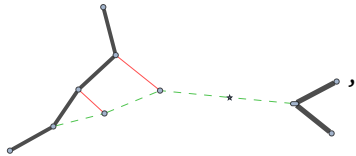

$$\begin{aligned}
& \frac{1}{r^3} G^3 m_2^3 \left( \frac{16 \hat{n} \cdot \vec{v}_1 \hat{n} \times \vec{a}_2 \cdot \vec{S}_1 - \frac{16}{3} \vec{a}_2 \times \vec{S}_1 \cdot \vec{v}_1 + 16 \hat{n} \cdot \vec{v}_2 \hat{n} \times \vec{S}_1 \cdot \vec{v}_2}{\epsilon_d} - 48 \log\left(\frac{r}{R_\theta}\right) \hat{n} \cdot \vec{v}_1 \hat{n} \times \vec{a}_2 \cdot \vec{S}_1 + \right. \\
& \left. 16 \hat{n} \cdot \vec{v}_1 \hat{n} \times \vec{a}_2 \cdot \vec{S}_1 + 16 \log\left(\frac{r}{R_\theta}\right) \vec{a}_2 \times \vec{S}_1 \cdot \vec{v}_1 - 48 \log\left(\frac{r}{R_\theta}\right) \hat{n} \cdot \vec{v}_2 \hat{n} \times \vec{S}_1 \cdot \vec{v}_2 + 16 \hat{n} \cdot \vec{v}_2 \hat{n} \times \vec{S}_1 \cdot \vec{v}_2 \right) + \\
& \frac{G^3 m_2^3 \left( 16 \log\left(\frac{r}{R_\theta}\right) \hat{n} \times \vec{a}_2 \cdot \vec{S}_1 - \frac{16 \hat{n} \times \vec{a}_2 \cdot \vec{S}_1}{3 \epsilon_d} \right)}{r^2} + \frac{1}{r^4} \\
& G^3 m_2^3 \left( \frac{-16 \hat{n} \cdot \vec{v}_2 \vec{S}_1 \times \vec{v}_1 \cdot \vec{v}_2 - 80 \hat{n} \cdot \vec{v}_1 \hat{n} \cdot \vec{v}_2 \hat{n} \times \vec{S}_1 \cdot \vec{v}_2 + 16 \vec{v}_1 \cdot \vec{v}_2 \hat{n} \times \vec{S}_1 \cdot \vec{v}_2}{\epsilon_d} + \right. \\
& 48 \log\left(\frac{r}{R_\theta}\right) \hat{n} \cdot \vec{v}_2 \vec{S}_1 \times \vec{v}_1 \cdot \vec{v}_2 + 240 \log\left(\frac{r}{R_\theta}\right) \hat{n} \cdot \vec{v}_1 \hat{n} \cdot \vec{v}_2 \hat{n} \times \vec{S}_1 \cdot \vec{v}_2 - 48 \log\left(\frac{r}{R_\theta}\right) \vec{v}_1 \cdot \vec{v}_2 \hat{n} \times \vec{S}_1 \cdot \vec{v}_2 - \\
& \left. 16 \hat{n} \cdot \vec{v}_2 \vec{S}_1 \times \vec{v}_1 \cdot \vec{v}_2 - 128 \hat{n} \cdot \vec{v}_1 \hat{n} \cdot \vec{v}_2 \hat{n} \times \vec{S}_1 \cdot \vec{v}_2 + 16 \vec{v}_1 \cdot \vec{v}_2 \hat{n} \times \vec{S}_1 \cdot \vec{v}_2 \right) \Bigg\}
\end{aligned}$$

{DiagSet[3, 1, 61],

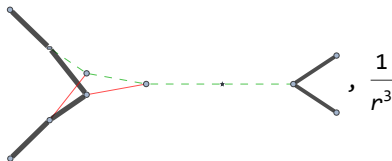

$$\begin{aligned}
& G^3 m_1^2 m_2 \left( \frac{-\frac{12}{5} \hat{n} \cdot \vec{v}_1 \hat{n} \times \vec{S}_1 \cdot \vec{a}_2 - \frac{4}{5} \vec{S}_1 \times \vec{v}_1 \cdot \vec{a}_2 + \frac{12}{5} \hat{n} \cdot \vec{v}_2 \hat{n} \times \vec{S}_1 \cdot \vec{v}_2}{\epsilon_d} + \frac{36}{5} \log\left(\frac{r}{R_\theta}\right) \hat{n} \cdot \vec{v}_1 \hat{n} \times \vec{S}_1 \cdot \vec{a}_2 - \frac{94}{25} \hat{n} \cdot \vec{v}_1 \hat{n} \times \vec{S}_1 \cdot \vec{a}_2 + \right. \\
& \left. \frac{12}{5} \log\left(\frac{r}{R_\theta}\right) \vec{S}_1 \times \vec{v}_1 \cdot \vec{a}_2 - \frac{34}{75} \vec{S}_1 \times \vec{v}_1 \cdot \vec{a}_2 - \frac{36}{5} \log\left(\frac{r}{R_\theta}\right) \hat{n} \cdot \vec{v}_2 \hat{n} \times \vec{S}_1 \cdot \vec{v}_2 + \frac{94}{25} \hat{n} \cdot \vec{v}_2 \hat{n} \times \vec{S}_1 \cdot \vec{v}_2 \right) +
\end{aligned}$$

$$\frac{G^3 m_1^2 m_2 \left( \frac{4 \hat{n} \cdot \vec{S}_1 \cdot \vec{a}_2}{5 \epsilon_d} - \frac{12}{5} \log \left( \frac{r}{R_\theta} \right) \hat{n} \times \vec{S}_1 \cdot \vec{a}_2 + \frac{34}{75} \hat{n} \times \vec{S}_1 \cdot \vec{a}_2 \right)}{r^2} + \frac{1}{r^4}$$

$$G^3 m_1^2 m_2 \left( \frac{-\frac{12}{5} \hat{n} \cdot \vec{v}_2 \vec{S}_1 \times \vec{v}_1 \cdot \vec{v}_2 - 12 \hat{n} \cdot \vec{v}_1 \hat{n} \cdot \vec{v}_2 \hat{n} \times \vec{S}_1 \cdot \vec{v}_2 + \frac{12}{5} \vec{v}_1 \cdot \vec{v}_2 \hat{n} \times \vec{S}_1 \cdot \vec{v}_2}{\epsilon_d} + \right.$$

$$\frac{36}{5} \log \left( \frac{r}{R_\theta} \right) \hat{n} \cdot \vec{v}_2 \vec{S}_1 \times \vec{v}_1 \cdot \vec{v}_2 + 36 \log \left( \frac{r}{R_\theta} \right) \hat{n} \cdot \vec{v}_1 \hat{n} \cdot \vec{v}_2 \hat{n} \times \vec{S}_1 \cdot \vec{v}_2 - \frac{36}{5} \log \left( \frac{r}{R_\theta} \right) \vec{v}_1 \cdot \vec{v}_2 \hat{n} \times \vec{S}_1 \cdot \vec{v}_2 -$$

$$\left. \frac{94}{25} \hat{n} \cdot \vec{v}_2 \vec{S}_1 \times \vec{v}_1 \cdot \vec{v}_2 - 26 \hat{n} \cdot \vec{v}_1 \hat{n} \cdot \vec{v}_2 \hat{n} \times \vec{S}_1 \cdot \vec{v}_2 + \frac{94}{25} \vec{v}_1 \cdot \vec{v}_2 \hat{n} \times \vec{S}_1 \cdot \vec{v}_2 \right\}$$

{DiagSet[3, 1, 62],

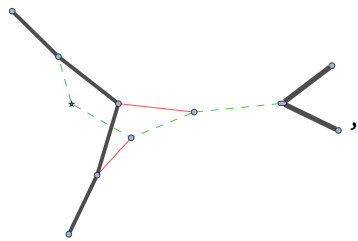

$$\frac{1}{r^3} G^3 m_2^3 \left( \frac{12 \hat{n} \cdot \vec{a}_2 \hat{n} \times \vec{S}_1 \cdot \vec{v}_2 + 12 \hat{n} \cdot \vec{v}_2 \hat{n} \times \vec{a}_2 \cdot \vec{S}_1 - 8 \vec{a}_2 \times \vec{S}_1 \cdot \vec{v}_2}{\epsilon_d} - 36 \log \left( \frac{r}{R_\theta} \right) \hat{n} \cdot \vec{a}_2 \hat{n} \times \vec{S}_1 \cdot \vec{v}_2 - \right.$$

$$36 \log \left( \frac{r}{R_\theta} \right) \hat{n} \cdot \vec{v}_2 \hat{n} \times \vec{a}_2 \cdot \vec{S}_1 + 4 \hat{n} \cdot \vec{a}_2 \hat{n} \times \vec{S}_1 \cdot \vec{v}_2 - 48 \hat{n} \cdot \vec{v}_1 \hat{n} \times \vec{a}_2 \cdot \vec{S}_1 + 36 \hat{n} \cdot \vec{v}_2 \hat{n} \times \vec{a}_2 \cdot \vec{S}_1 +$$

$$24 \log \left( \frac{r}{R_\theta} \right) \vec{a}_2 \times \vec{S}_1 \cdot \vec{v}_2 + 16 \vec{a}_2 \times \vec{S}_1 \cdot \vec{v}_1 - \frac{16}{3} \vec{a}_2 \times \vec{S}_1 \cdot \vec{v}_2 - 16 \hat{n} \cdot \vec{v}_2 \hat{n} \times \vec{S}_1 \cdot \vec{v}_2 \left. \right) + \frac{16 G^3 m_2^3 \hat{n} \times \vec{a}_2 \cdot \vec{S}_1}{r^2} + \frac{1}{r^4}$$

$$G^3 m_2^3 \left( -32 (\hat{n} \cdot \vec{v}_2)^2 \hat{n} \times \vec{S}_1 \cdot \vec{v}_2 + 16 \hat{n} \cdot \vec{v}_2 \vec{S}_1 \times \vec{v}_1 \cdot \vec{v}_2 + 80 \hat{n} \cdot \vec{v}_1 \hat{n} \cdot \vec{v}_2 \hat{n} \times \vec{S}_1 \cdot \vec{v}_2 - 16 \vec{v}_1 \cdot \vec{v}_2 \hat{n} \times \vec{S}_1 \cdot \vec{v}_2 \right) \}$$

{DiagSet[3, 1, 63],

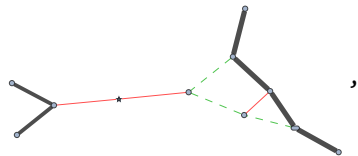

$$\frac{1}{r^3} G^3 m_1^2 m_2 \left( \frac{-\frac{4}{5} \hat{n} \cdot \vec{v}_2 \hat{n} \times \vec{S}_1 \cdot \vec{a}_1 + \frac{4}{15} \vec{S}_1 \times \vec{a}_1 \cdot \vec{v}_2 - \frac{4}{5} \hat{n} \cdot \vec{v}_2 \hat{n} \times \vec{S}_1 \cdot \vec{v}_1 + \frac{4}{15} \vec{S}_1 \times \vec{v}_1 \cdot \vec{v}_2}{\epsilon_d} + \right.$$

$$\frac{12}{5} \log \left( \frac{r}{R_\theta} \right) \hat{n} \cdot \vec{v}_2 \hat{n} \times \vec{S}_1 \cdot \vec{a}_1 - \frac{38}{25} \hat{n} \cdot \vec{v}_2 \hat{n} \times \vec{S}_1 \cdot \vec{a}_1 - \frac{4}{5} \log \left( \frac{r}{R_\theta} \right) \vec{S}_1 \times \vec{a}_1 \cdot \vec{v}_2 + \frac{6}{25} \vec{S}_1 \times \vec{a}_1 \cdot \vec{v}_2 +$$

$$\left. \frac{12}{5} \log \left( \frac{r}{R_\theta} \right) \hat{n} \cdot \vec{v}_2 \hat{n} \times \vec{S}_1 \cdot \vec{v}_1 - \frac{38}{25} \hat{n} \cdot \vec{v}_2 \hat{n} \times \vec{S}_1 \cdot \vec{v}_1 - \frac{4}{5} \log \left( \frac{r}{R_\theta} \right) \vec{S}_1 \times \vec{v}_1 \cdot \vec{v}_2 + \frac{6}{25} \vec{S}_1 \times \vec{v}_1 \cdot \vec{v}_2 \right) +$$

$$\frac{1}{r^4} G^3 m_1^2 m_2 \left( \frac{-\frac{4}{5} \hat{n} \cdot \vec{v}_1 \vec{S}_1 \times \vec{v}_1 \cdot \vec{v}_2 + 4 \hat{n} \cdot \vec{v}_2 \hat{n} \cdot \vec{v}_1 \hat{n} \times \vec{S}_1 \cdot \vec{v}_1 - \frac{4}{5} \vec{v}_1 \cdot \vec{v}_2 \hat{n} \times \vec{S}_1 \cdot \vec{v}_1}{\epsilon_d} + \right.$$

$$\frac{12}{5} \log \left( \frac{r}{R_\theta} \right) \hat{n} \cdot \vec{v}_1 \vec{S}_1 \times \vec{v}_1 \cdot \vec{v}_2 - 12 \log \left( \frac{r}{R_\theta} \right) \hat{n} \cdot \vec{v}_2 \hat{n} \cdot \vec{v}_1 \hat{n} \times \vec{S}_1 \cdot \vec{v}_1 + \frac{12}{5} \log \left( \frac{r}{R_\theta} \right) \vec{v}_1 \cdot \vec{v}_2 \hat{n} \times \vec{S}_1 \cdot \vec{v}_1 -$$

$$\left. \frac{38}{25} \hat{n} \cdot \vec{v}_1 \vec{S}_1 \times \vec{v}_1 \cdot \vec{v}_2 + 10 \hat{n} \cdot \vec{v}_2 \hat{n} \cdot \vec{v}_1 \hat{n} \times \vec{S}_1 \cdot \vec{v}_1 - \frac{38}{25} \vec{v}_1 \cdot \vec{v}_2 \hat{n} \times \vec{S}_1 \cdot \vec{v}_1 \right\}$$

{DiagSet[3, 1, 64],

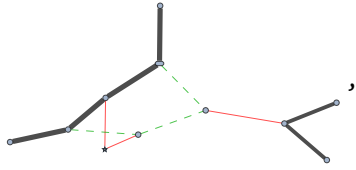

$$\frac{1}{r^3} G^3 m_1^2 m_2 \left( \frac{\frac{4}{5} \hat{n} \cdot \vec{a}_1 \hat{n} \times \vec{S}_1 \cdot \vec{v}_1 - \frac{12}{5} \hat{n} \cdot \vec{v}_1 \hat{n} \times \vec{S}_1 \cdot \vec{a}_1 - \frac{16}{15} \vec{S}_1 \times \vec{v}_1 \cdot \vec{a}_1 - \frac{8}{5} \hat{n} \cdot \vec{v}_1 \hat{n} \times \vec{S}_1 \cdot \vec{v}_1}{\epsilon_d} - \right.$$

$$\frac{12}{5} \log\left(\frac{r}{R_\theta}\right) \hat{n} \cdot \vec{a}_1 \hat{n} \times \vec{S}_1 \cdot \vec{v}_1 + \frac{36}{5} \log\left(\frac{r}{R_\theta}\right) \hat{n} \cdot \vec{v}_1 \hat{n} \times \vec{S}_1 \cdot \vec{a}_1 + \frac{28}{25} \hat{n} \cdot \vec{a}_1 \hat{n} \times \vec{S}_1 \cdot \vec{v}_1 - \frac{124}{25} \hat{n} \cdot \vec{v}_1 \hat{n} \times \vec{S}_1 \cdot \vec{a}_1 +$$

$$\left. \frac{16}{5} \log\left(\frac{r}{R_\theta}\right) \vec{S}_1 \times \vec{v}_1 \cdot \vec{a}_1 - \frac{64}{25} \vec{S}_1 \times \vec{v}_1 \cdot \vec{a}_1 + \frac{24}{5} \log\left(\frac{r}{R_\theta}\right) \hat{n} \cdot \vec{v}_1 \hat{n} \times \vec{S}_1 \cdot \vec{v}_1 - \frac{96}{25} \hat{n} \cdot \vec{v}_1 \hat{n} \times \vec{S}_1 \cdot \vec{v}_1 \right) + \frac{1}{r^4}$$

$$G^3 m_1^2 m_2 \left( \frac{1}{\epsilon_d} \left( \frac{48}{7} (\hat{n} \cdot \vec{v}_1)^2 \hat{n} \times \vec{S}_1 \cdot \vec{v}_1 + \frac{8}{5} \hat{n} \cdot \vec{v}_1 \vec{S}_1 \times \vec{v}_1 \cdot \vec{v}_2 - 8 \hat{n} \cdot \vec{v}_2 \hat{n} \cdot \vec{v}_1 \hat{n} \times \vec{S}_1 \cdot \vec{v}_1 - \frac{48}{35} \vec{v}_1 \cdot \vec{v}_1 \hat{n} \times \vec{S}_1 \cdot \vec{v}_1 + \right.$$

$$\frac{8}{5} \vec{v}_1 \cdot \vec{v}_2 \hat{n} \times \vec{S}_1 \cdot \vec{v}_1 \right) - \frac{144}{7} \log\left(\frac{r}{R_\theta}\right) (\hat{n} \cdot \vec{v}_1)^2 \hat{n} \times \vec{S}_1 \cdot \vec{v}_1 - \frac{24}{5} \log\left(\frac{r}{R_\theta}\right) \hat{n} \cdot \vec{v}_1 \vec{S}_1 \times \vec{v}_1 \cdot \vec{v}_2 + 24 \log\left(\frac{r}{R_\theta}\right) \hat{n} \cdot \vec{v}_2$$

$$\hat{n} \cdot \vec{v}_1 \hat{n} \times \vec{S}_1 \cdot \vec{v}_1 + \frac{144}{35} \log\left(\frac{r}{R_\theta}\right) \vec{v}_1 \cdot \vec{v}_1 \hat{n} \times \vec{S}_1 \cdot \vec{v}_1 - \frac{24}{5} \log\left(\frac{r}{R_\theta}\right) \vec{v}_1 \cdot \vec{v}_2 \hat{n} \times \vec{S}_1 \cdot \vec{v}_1 + \frac{976}{49} (\hat{n} \cdot \vec{v}_1)^2 \hat{n} \times \vec{S}_1 \cdot \vec{v}_1 +$$

$$\left. \frac{96}{25} \hat{n} \cdot \vec{v}_1 \vec{S}_1 \times \vec{v}_1 \cdot \vec{v}_2 - 24 \hat{n} \cdot \vec{v}_2 \hat{n} \cdot \vec{v}_1 \hat{n} \times \vec{S}_1 \cdot \vec{v}_1 - \frac{2192 \vec{v}_1 \cdot \vec{v}_1 \hat{n} \times \vec{S}_1 \cdot \vec{v}_1}{1225} + \frac{96}{25} \vec{v}_1 \cdot \vec{v}_2 \hat{n} \times \vec{S}_1 \cdot \vec{v}_1 \right\}$$

{DiagSet[3, 1, 65],

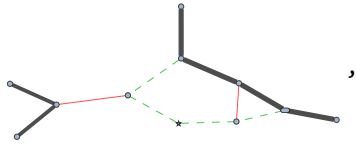

$$\frac{1}{r^3} G^3 m_1^2 m_2 \left( \frac{\frac{4}{5} \hat{n} \cdot \vec{a}_1 \hat{n} \times \vec{S}_1 \cdot \vec{v}_1 - \frac{4}{5} \hat{n} \cdot \vec{v}_1 \hat{n} \times \vec{S}_1 \cdot \vec{a}_1 - \frac{8}{15} \vec{S}_1 \times \vec{v}_1 \cdot \vec{a}_1}{\epsilon_d} - \frac{12}{5} \log\left(\frac{r}{R_\theta}\right) \hat{n} \cdot \vec{a}_1 \hat{n} \times \vec{S}_1 \cdot \vec{v}_1 + \right.$$

$$\frac{12}{5} \log\left(\frac{r}{R_\theta}\right) \hat{n} \cdot \vec{v}_1 \hat{n} \times \vec{S}_1 \cdot \vec{a}_1 + \frac{58}{25} \hat{n} \cdot \vec{a}_1 \hat{n} \times \vec{S}_1 \cdot \vec{v}_1 - \frac{98}{25} \hat{n} \cdot \vec{v}_1 \hat{n} \times \vec{S}_1 \cdot \vec{a}_1 + \frac{8}{5} \log\left(\frac{r}{R_\theta}\right) \vec{S}_1 \times \vec{v}_1 \cdot \vec{a}_1 -$$

$$\left. \frac{176}{75} \vec{S}_1 \times \vec{v}_1 \cdot \vec{a}_1 - \frac{12}{5} \hat{n} \cdot \vec{v}_1 \hat{n} \times \vec{S}_1 \cdot \vec{v}_1 + 4 \hat{n} \cdot \vec{v}_2 \hat{n} \times \vec{S}_1 \cdot \vec{v}_1 - \frac{4}{3} \vec{S}_1 \times \vec{v}_1 \cdot \vec{v}_2 \right) + \frac{4 G^3 m_1^2 m_2 \hat{n} \times \vec{S}_1 \cdot \vec{a}_1}{3 r^2} + \frac{1}{r^4} G^3 m_1^2 m_2$$

$$\left( \frac{24}{7} (\hat{n} \cdot \vec{v}_1)^2 \hat{n} \times \vec{S}_1 \cdot \vec{v}_1 + \frac{8}{5} \hat{n} \cdot \vec{v}_1 \vec{S}_1 \times \vec{v}_1 \cdot \vec{v}_2 - 8 \hat{n} \cdot \vec{v}_2 \hat{n} \cdot \vec{v}_1 \hat{n} \times \vec{S}_1 \cdot \vec{v}_1 - \frac{24}{35} \vec{v}_1 \cdot \vec{v}_1 \hat{n} \times \vec{S}_1 \cdot \vec{v}_1 + \frac{8}{5} \vec{v}_1 \cdot \vec{v}_2 \hat{n} \times \vec{S}_1 \cdot \vec{v}_1 \right\}$$

{DiagSet[3, 1, 66],

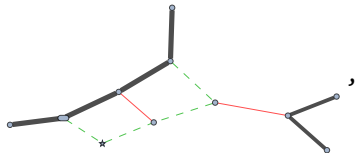

$$\frac{8 \hat{n} \times \vec{S}_1 \cdot \vec{a}_1 m_1^2 m_2 G^3}{r^2} + \frac{1}{r^3} m_1^2 m_2 \left( -8 \vec{S}_1 \times \vec{v}_1 \cdot \vec{v}_2 - \frac{159}{25} \vec{S}_1 \times \vec{v}_1 \cdot \vec{a}_1 + \frac{143}{25} \hat{n} \times \vec{S}_1 \cdot \vec{v}_1 \hat{n} \cdot \vec{a}_1 - \right.$$

$$\left. \frac{499}{25} \hat{n} \times \vec{S}_1 \cdot \vec{v}_1 \hat{n} \cdot \vec{v}_1 - \frac{244}{25} \hat{n} \times \vec{S}_1 \cdot \vec{a}_1 \hat{n} \cdot \vec{v}_1 + 24 \hat{n} \times \vec{S}_1 \cdot \vec{v}_1 \hat{n} \cdot \vec{v}_2 + \frac{26}{5} \vec{S}_1 \times \vec{v}_1 \cdot \vec{a}_1 \log\left(\frac{r}{R_\theta}\right) - \right.$$

$$\frac{42}{5} \hat{n} \times \vec{S}_1 \cdot \vec{v}_1 \hat{n} \cdot \vec{a}_1 \log\left(\frac{r}{R_0}\right) + \frac{6}{5} \hat{n} \times \vec{S}_1 \cdot \vec{v}_1 \hat{n} \cdot \vec{v}_1 \log\left(\frac{r}{R_0}\right) + \frac{36}{5} \hat{n} \times \vec{S}_1 \cdot \vec{a}_1 \hat{n} \cdot \vec{v}_1 \log\left(\frac{r}{R_0}\right) +$$

$$\frac{-\frac{26}{15} \vec{S}_1 \times \vec{v}_1 \cdot \vec{a}_1 + \frac{14}{5} \hat{n} \times \vec{S}_1 \cdot \vec{v}_1 \hat{n} \cdot \vec{a}_1 - \frac{2}{5} \hat{n} \times \vec{S}_1 \cdot \vec{v}_1 \hat{n} \cdot \vec{v}_1 - \frac{12}{5} \hat{n} \times \vec{S}_1 \cdot \vec{a}_1 \hat{n} \cdot \vec{v}_1}{\epsilon_d} \left) G^3 + \frac{1}{r^4} \right.$$

$$m_1^2 m_2 \left( \frac{571}{49} \hat{n} \times \vec{S}_1 \cdot \vec{v}_1 (\hat{n} \cdot \vec{v}_1)^2 + \frac{18}{7} \hat{n} \times \vec{S}_1 \cdot \vec{v}_1 \log\left(\frac{r}{R_0}\right) (\hat{n} \cdot \vec{v}_1)^2 + \frac{101}{25} \vec{S}_1 \times \vec{v}_1 \cdot \vec{v}_2 \hat{n} \cdot \vec{v}_1 - 19 \hat{n} \times \vec{S}_1 \cdot \vec{v}_1 \hat{n} \cdot \vec{v}_2 \hat{n} \cdot \vec{v}_1 + \right.$$

$$\frac{6}{5} \vec{S}_1 \times \vec{v}_1 \cdot \vec{v}_2 \log\left(\frac{r}{R_0}\right) \hat{n} \cdot \vec{v}_1 - 6 \hat{n} \times \vec{S}_1 \cdot \vec{v}_1 \hat{n} \cdot \vec{v}_2 \log\left(\frac{r}{R_0}\right) \hat{n} \cdot \vec{v}_1 - \frac{4661 \hat{n} \times \vec{S}_1 \cdot \vec{v}_1 \vec{v}_1 \cdot \vec{v}_1}{1225} + \frac{101}{25} \hat{n} \times \vec{S}_1 \cdot \vec{v}_1 \vec{v}_1 \cdot \vec{v}_2 -$$

$$\frac{18}{35} \hat{n} \times \vec{S}_1 \cdot \vec{v}_1 \vec{v}_1 \cdot \vec{v}_1 \log\left(\frac{r}{R_0}\right) + \frac{6}{5} \hat{n} \times \vec{S}_1 \cdot \vec{v}_1 \vec{v}_1 \cdot \vec{v}_2 \log\left(\frac{r}{R_0}\right) + \frac{1}{\epsilon_d} \left( -\frac{6}{7} \hat{n} \times \vec{S}_1 \cdot \vec{v}_1 (\hat{n} \cdot \vec{v}_1)^2 - \right.$$

$$\left. \left. \frac{2}{5} \vec{S}_1 \times \vec{v}_1 \cdot \vec{v}_2 \hat{n} \cdot \vec{v}_1 + 2 \hat{n} \times \vec{S}_1 \cdot \vec{v}_1 \hat{n} \cdot \vec{v}_2 \hat{n} \cdot \vec{v}_1 + \frac{6}{35} \hat{n} \times \vec{S}_1 \cdot \vec{v}_1 \vec{v}_1 \cdot \vec{v}_1 - \frac{2}{5} \hat{n} \times \vec{S}_1 \cdot \vec{v}_1 \vec{v}_1 \cdot \vec{v}_2 \right) \right) G^3 \}$$

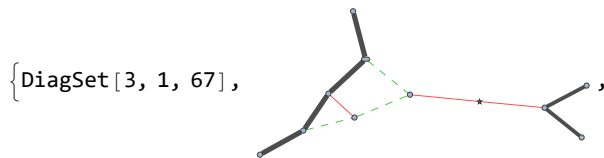

$$\frac{1}{r^3} G^3 m_1^2 m_2 \left( \frac{-\frac{8}{5} \hat{n} \cdot \vec{v}_2 \hat{n} \times \vec{S}_1 \cdot \vec{a}_1 + \frac{8}{15} \vec{S}_1 \times \vec{a}_1 \cdot \vec{v}_2 - \frac{8}{5} \hat{n} \cdot \vec{v}_2 \hat{n} \times \vec{S}_1 \cdot \vec{v}_1 + \frac{8}{15} \vec{S}_1 \times \vec{v}_1 \cdot \vec{v}_2}{\epsilon_d} + \right.$$

$$\frac{24}{5} \log\left(\frac{r}{R_0}\right) \hat{n} \cdot \vec{v}_2 \hat{n} \times \vec{S}_1 \cdot \vec{a}_1 - \frac{56}{25} \hat{n} \cdot \vec{v}_2 \hat{n} \times \vec{S}_1 \cdot \vec{a}_1 - \frac{8}{5} \log\left(\frac{r}{R_0}\right) \vec{S}_1 \times \vec{a}_1 \cdot \vec{v}_2 + \frac{16}{75} \vec{S}_1 \times \vec{a}_1 \cdot \vec{v}_2 +$$

$$\left. \frac{24}{5} \log\left(\frac{r}{R_0}\right) \hat{n} \cdot \vec{v}_2 \hat{n} \times \vec{S}_1 \cdot \vec{v}_1 - \frac{56}{25} \hat{n} \cdot \vec{v}_2 \hat{n} \times \vec{S}_1 \cdot \vec{v}_1 - \frac{8}{5} \log\left(\frac{r}{R_0}\right) \vec{S}_1 \times \vec{v}_1 \cdot \vec{v}_2 + \frac{16}{75} \vec{S}_1 \times \vec{v}_1 \cdot \vec{v}_2 \right) +$$

$$\frac{1}{r^4} G^3 m_1^2 m_2 \left( \frac{-\frac{8}{5} \hat{n} \cdot \vec{v}_1 \vec{S}_1 \times \vec{v}_1 \cdot \vec{v}_2 + 8 \hat{n} \cdot \vec{v}_2 \hat{n} \cdot \vec{v}_1 \hat{n} \times \vec{S}_1 \cdot \vec{v}_1 - \frac{8}{5} \vec{v}_1 \cdot \vec{v}_2 \hat{n} \times \vec{S}_1 \cdot \vec{v}_1}{\epsilon_d} + \right.$$

$$\frac{24}{5} \log\left(\frac{r}{R_0}\right) \hat{n} \cdot \vec{v}_1 \vec{S}_1 \times \vec{v}_1 \cdot \vec{v}_2 - 24 \log\left(\frac{r}{R_0}\right) \hat{n} \cdot \vec{v}_2 \hat{n} \cdot \vec{v}_1 \hat{n} \times \vec{S}_1 \cdot \vec{v}_1 + \frac{24}{5} \log\left(\frac{r}{R_0}\right) \vec{v}_1 \cdot \vec{v}_2 \hat{n} \times \vec{S}_1 \cdot \vec{v}_1 -$$

$$\left. \frac{56}{25} \hat{n} \cdot \vec{v}_1 \vec{S}_1 \times \vec{v}_1 \cdot \vec{v}_2 + 16 \hat{n} \cdot \vec{v}_2 \hat{n} \cdot \vec{v}_1 \hat{n} \times \vec{S}_1 \cdot \vec{v}_1 - \frac{56}{25} \vec{v}_1 \cdot \vec{v}_2 \hat{n} \times \vec{S}_1 \cdot \vec{v}_1 \right) \}$$

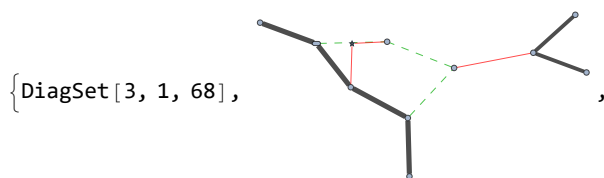

$$\frac{1}{r^3} G^3 m_1^2 m_2 \left( \frac{-\frac{2}{5} \hat{n} \cdot \vec{a}_1 \hat{n} \times \vec{S}_1 \cdot \vec{v}_1 - \frac{4}{5} \hat{n} \cdot \vec{v}_1 \hat{n} \times \vec{S}_1 \cdot \vec{a}_1 - \frac{2}{15} \vec{S}_1 \times \vec{v}_1 \cdot \vec{a}_1 - \frac{6}{5} \hat{n} \cdot \vec{v}_1 \hat{n} \times \vec{S}_1 \cdot \vec{v}_1}{\epsilon_d} + \right.$$

$$\frac{6}{5} \log\left(\frac{r}{R_0}\right) \hat{n} \cdot \vec{a}_1 \hat{n} \times \vec{S}_1 \cdot \vec{v}_1 + \frac{12}{5} \log\left(\frac{r}{R_0}\right) \hat{n} \cdot \vec{v}_1 \hat{n} \times \vec{S}_1 \cdot \vec{a}_1 - \frac{9}{25} \hat{n} \cdot \vec{a}_1 \hat{n} \times \vec{S}_1 \cdot \vec{v}_1 - \frac{68}{25} \hat{n} \cdot \vec{v}_1 \hat{n} \times \vec{S}_1 \cdot \vec{a}_1 +$$

$$\frac{2}{5} \log\left(\frac{r}{R_0}\right) \vec{S}_1 \times \vec{v}_1 \cdot \vec{a}_1 + \frac{11}{75} \vec{S}_1 \times \vec{v}_1 \cdot \vec{a}_1 + \frac{18}{5} \log\left(\frac{r}{R_0}\right) \hat{n} \cdot \vec{v}_1 \hat{n} \times \vec{S}_1 \cdot \vec{v}_1 - \frac{77}{25} \hat{n} \cdot \vec{v}_1 \hat{n} \times \vec{S}_1 \cdot \vec{v}_1 \left. \right\} + \frac{1}{r^4}$$

$$G^3 m_1^2 m_2 \left( \frac{1}{\epsilon_d} \left( \frac{34}{7} (\hat{n} \cdot \vec{v}_1)^2 \hat{n} \times \vec{S}_1 \cdot \vec{v}_1 + \frac{6}{5} \hat{n} \cdot \vec{v}_1 \vec{S}_1 \times \vec{v}_1 \cdot \vec{v}_2 - 6 \hat{n} \cdot \vec{v}_2 \hat{n} \cdot \vec{v}_1 \hat{n} \times \vec{S}_1 \cdot \vec{v}_1 - \frac{34}{35} \vec{v}_1 \cdot \vec{v}_1 \hat{n} \times \vec{S}_1 \cdot \vec{v}_1 + \right. \right. \\ \left. \frac{6}{5} \vec{v}_1 \cdot \vec{v}_2 \hat{n} \times \vec{S}_1 \cdot \vec{v}_1 \right) - \frac{102}{7} \log\left(\frac{r}{R_0}\right) (\hat{n} \cdot \vec{v}_1)^2 \hat{n} \times \vec{S}_1 \cdot \vec{v}_1 - \frac{18}{5} \log\left(\frac{r}{R_0}\right) \hat{n} \cdot \vec{v}_1 \vec{S}_1 \times \vec{v}_1 \cdot \vec{v}_2 + 18 \log\left(\frac{r}{R_0}\right) \hat{n} \cdot \vec{v}_2 \\ \hat{n} \cdot \vec{v}_1 \hat{n} \times \vec{S}_1 \cdot \vec{v}_1 + \frac{102}{35} \log\left(\frac{r}{R_0}\right) \vec{v}_1 \cdot \vec{v}_1 \hat{n} \times \vec{S}_1 \cdot \vec{v}_1 - \frac{18}{5} \log\left(\frac{r}{R_0}\right) \vec{v}_1 \cdot \vec{v}_2 \hat{n} \times \vec{S}_1 \cdot \vec{v}_1 + \frac{731}{49} (\hat{n} \cdot \vec{v}_1)^2 \hat{n} \times \vec{S}_1 \cdot \vec{v}_1 + \\ \left. \frac{77}{25} \hat{n} \cdot \vec{v}_1 \vec{S}_1 \times \vec{v}_1 \cdot \vec{v}_2 - 19 \hat{n} \cdot \vec{v}_2 \hat{n} \cdot \vec{v}_1 \hat{n} \times \vec{S}_1 \cdot \vec{v}_1 - \frac{2241 \vec{v}_1 \cdot \vec{v}_1 \hat{n} \times \vec{S}_1 \cdot \vec{v}_1}{1225} + \frac{77}{25} \vec{v}_1 \cdot \vec{v}_2 \hat{n} \times \vec{S}_1 \cdot \vec{v}_1 \right) \Bigg\}$$

{DiagSet[3, 1, 69], 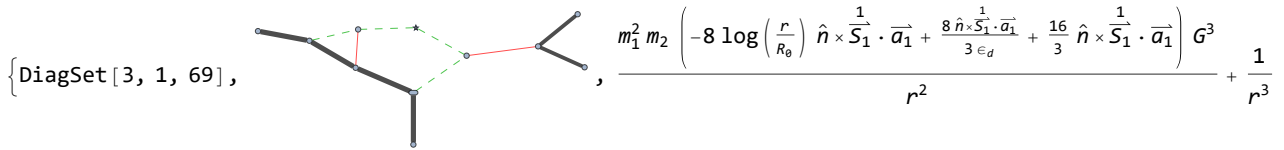,  $\frac{m_1^2 m_2 \left( -8 \log\left(\frac{r}{R_0}\right) \hat{n} \times \vec{S}_1 \cdot \vec{a}_1 + \frac{8 \hat{n} \times \vec{S}_1 \cdot \vec{a}_1}{3 \epsilon_d} + \frac{16}{3} \hat{n} \times \vec{S}_1 \cdot \vec{a}_1 \right) G^3}{r^2} + \frac{1}{r^3}$

$$m_1^2 m_2 \left( 8 \log\left(\frac{r}{R_0}\right) \vec{S}_1 \times \vec{a}_1 \cdot \vec{v}_2 - \frac{16}{3} \vec{S}_1 \times \vec{a}_1 \cdot \vec{v}_2 - \frac{208}{25} \vec{S}_1 \times \vec{v}_1 \cdot \vec{a}_1 + \frac{208}{25} \hat{n} \times \vec{S}_1 \cdot \vec{v}_1 \hat{n} \cdot \vec{a}_1 - \frac{272}{25} \hat{n} \times \vec{S}_1 \cdot \vec{v}_1 \hat{n} \cdot \vec{v}_1 - \right. \\ \left. \frac{536}{25} \hat{n} \times \vec{S}_1 \cdot \vec{a}_1 \hat{n} \cdot \vec{v}_1 + 24 \hat{n} \times \vec{S}_1 \cdot \vec{a}_1 \hat{n} \cdot \vec{v}_2 + \frac{72}{5} \vec{S}_1 \times \vec{v}_1 \cdot \vec{a}_1 \log\left(\frac{r}{R_0}\right) - \frac{72}{5} \hat{n} \times \vec{S}_1 \cdot \vec{v}_1 \hat{n} \cdot \vec{a}_1 \log\left(\frac{r}{R_0}\right) + \right. \\ \left. \frac{48}{5} \hat{n} \times \vec{S}_1 \cdot \vec{v}_1 \hat{n} \cdot \vec{v}_1 \log\left(\frac{r}{R_0}\right) + \frac{144}{5} \hat{n} \times \vec{S}_1 \cdot \vec{a}_1 \hat{n} \cdot \vec{v}_1 \log\left(\frac{r}{R_0}\right) - 24 \hat{n} \times \vec{S}_1 \cdot \vec{a}_1 \hat{n} \cdot \vec{v}_2 \log\left(\frac{r}{R_0}\right) + \frac{1}{\epsilon_d} \left( -\frac{8}{3} \vec{S}_1 \times \vec{a}_1 \cdot \vec{v}_2 - \right. \right. \\ \left. \frac{24}{5} \vec{S}_1 \times \vec{v}_1 \cdot \vec{a}_1 + \frac{24}{5} \hat{n} \times \vec{S}_1 \cdot \vec{v}_1 \hat{n} \cdot \vec{a}_1 - \frac{16}{5} \hat{n} \times \vec{S}_1 \cdot \vec{v}_1 \hat{n} \cdot \vec{v}_1 - \frac{48}{5} \hat{n} \times \vec{S}_1 \cdot \vec{a}_1 \hat{n} \cdot \vec{v}_1 + 8 \hat{n} \times \vec{S}_1 \cdot \vec{a}_1 \hat{n} \cdot \vec{v}_2 \right) \Bigg) G^3 + \\ \frac{1}{r^4} m_1^2 m_2 \left( \frac{1312}{49} \hat{n} \times \vec{S}_1 \cdot \vec{v}_1 (\hat{n} \cdot \vec{v}_1)^2 - \frac{144}{7} \hat{n} \times \vec{S}_1 \cdot \vec{v}_1 \log\left(\frac{r}{R_0}\right) (\hat{n} \cdot \vec{v}_1)^2 + \frac{272}{25} \vec{S}_1 \times \vec{v}_1 \cdot \vec{v}_2 \hat{n} \cdot \vec{v}_1 - \right. \\ \left. 64 \hat{n} \times \vec{S}_1 \cdot \vec{v}_1 \hat{n} \cdot \vec{v}_2 \hat{n} \cdot \vec{v}_1 - \frac{48}{5} \vec{S}_1 \times \vec{v}_1 \cdot \vec{v}_2 \log\left(\frac{r}{R_0}\right) \hat{n} \cdot \vec{v}_1 + 48 \hat{n} \times \vec{S}_1 \cdot \vec{v}_1 \hat{n} \cdot \vec{v}_2 \log\left(\frac{r}{R_0}\right) \hat{n} \cdot \vec{v}_1 - \right. \\ \left. \frac{3872 \hat{n} \times \vec{S}_1 \cdot \vec{v}_1 \vec{v}_1 \cdot \vec{v}_1}{1225} + \frac{272}{25} \hat{n} \times \vec{S}_1 \cdot \vec{v}_1 \vec{v}_1 \cdot \vec{v}_2 + \frac{144}{35} \hat{n} \times \vec{S}_1 \cdot \vec{v}_1 \vec{v}_1 \cdot \vec{v}_1 \log\left(\frac{r}{R_0}\right) - \right. \\ \left. \frac{48}{5} \hat{n} \times \vec{S}_1 \cdot \vec{v}_1 \vec{v}_1 \cdot \vec{v}_2 \log\left(\frac{r}{R_0}\right) + \frac{1}{\epsilon_d} \left( \frac{48}{7} \hat{n} \times \vec{S}_1 \cdot \vec{v}_1 (\hat{n} \cdot \vec{v}_1)^2 + \frac{16}{5} \vec{S}_1 \times \vec{v}_1 \cdot \vec{v}_2 \hat{n} \cdot \vec{v}_1 - \right. \right. \\ \left. \left. 16 \hat{n} \times \vec{S}_1 \cdot \vec{v}_1 \hat{n} \cdot \vec{v}_2 \hat{n} \cdot \vec{v}_1 - \frac{48}{35} \hat{n} \times \vec{S}_1 \cdot \vec{v}_1 \vec{v}_1 \cdot \vec{v}_1 + \frac{16}{5} \hat{n} \times \vec{S}_1 \cdot \vec{v}_1 \vec{v}_1 \cdot \vec{v}_2 \right) \right) \Bigg\} G^3 \Bigg\}$$

{DiagSet[3, 1, 70], 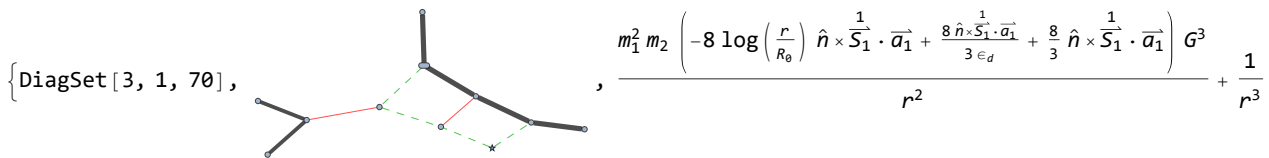,  $\frac{m_1^2 m_2 \left( -8 \log\left(\frac{r}{R_0}\right) \hat{n} \times \vec{S}_1 \cdot \vec{a}_1 + \frac{8 \hat{n} \times \vec{S}_1 \cdot \vec{a}_1}{3 \epsilon_d} + \frac{8}{3} \hat{n} \times \vec{S}_1 \cdot \vec{a}_1 \right) G^3}{r^2} + \frac{1}{r^3}$

$$m_1^2 m_2 \left( 8 \log\left(\frac{r}{R_0}\right) \vec{S}_1 \times \vec{a}_1 \cdot \vec{v}_2 - \frac{8}{3} \vec{S}_1 \times \vec{a}_1 \cdot \vec{v}_2 - \frac{152}{25} \vec{S}_1 \times \vec{v}_1 \cdot \vec{a}_1 + \frac{116}{25} \hat{n} \times \vec{S}_1 \cdot \vec{v}_1 \hat{n} \cdot \vec{a}_1 - \frac{96}{25} \hat{n} \times \vec{S}_1 \cdot \vec{v}_1 \hat{n} \cdot \vec{v}_1 - \right. \\ \left. \frac{84}{5} \hat{n} \times \vec{S}_1 \cdot \vec{a}_1 \hat{n} \cdot \vec{v}_1 + 16 \hat{n} \times \vec{S}_1 \cdot \vec{a}_1 \hat{n} \cdot \vec{v}_2 + \frac{88}{5} \vec{S}_1 \times \vec{v}_1 \cdot \vec{a}_1 \log\left(\frac{r}{R_0}\right) - \frac{84}{5} \hat{n} \times \vec{S}_1 \cdot \vec{v}_1 \hat{n} \cdot \vec{a}_1 \log\left(\frac{r}{R_0}\right) + \right. \\ \left. \frac{24}{5} \hat{n} \times \vec{S}_1 \cdot \vec{v}_1 \hat{n} \cdot \vec{v}_1 \log\left(\frac{r}{R_0}\right) + 36 \hat{n} \times \vec{S}_1 \cdot \vec{a}_1 \hat{n} \cdot \vec{v}_1 \log\left(\frac{r}{R_0}\right) - 24 \hat{n} \times \vec{S}_1 \cdot \vec{a}_1 \hat{n} \cdot \vec{v}_2 \log\left(\frac{r}{R_0}\right) + \frac{1}{\epsilon_d} \left( -\frac{8}{3} \vec{S}_1 \times \vec{a}_1 \cdot \vec{v}_2 - \right. \right. \\ \left. \frac{88}{15} \vec{S}_1 \times \vec{v}_1 \cdot \vec{a}_1 + \frac{28}{5} \hat{n} \times \vec{S}_1 \cdot \vec{v}_1 \hat{n} \cdot \vec{a}_1 - \frac{8}{5} \hat{n} \times \vec{S}_1 \cdot \vec{v}_1 \hat{n} \cdot \vec{v}_1 - 12 \hat{n} \times \vec{S}_1 \cdot \vec{a}_1 \hat{n} \cdot \vec{v}_1 + 8 \hat{n} \times \vec{S}_1 \cdot \vec{a}_1 \hat{n} \cdot \vec{v}_2 \right) \Bigg) G^3 + \frac{1}{r^4}$$

$$m_1^2 m_2 \left( \frac{688}{49} \hat{n} \times \vec{S}_1 \cdot \vec{v}_1 (\hat{n} \cdot \vec{v}_1)^2 - \frac{96}{7} \hat{n} \times \vec{S}_1 \cdot \vec{v}_1 \log\left(\frac{r}{R_\theta}\right) (\hat{n} \cdot \vec{v}_1)^2 + \frac{96}{25} \vec{S}_1 \times \vec{v}_1 \cdot \vec{v}_2 \hat{n} \cdot \vec{v}_1 - 24 \hat{n} \times \vec{S}_1 \cdot \vec{v}_1 \hat{n} \cdot \vec{v}_2 \hat{n} \cdot \vec{v}_1 - \right. \\ \left. \frac{24}{5} \vec{S}_1 \times \vec{v}_1 \cdot \vec{v}_2 \log\left(\frac{r}{R_\theta}\right) \hat{n} \cdot \vec{v}_1 + 24 \hat{n} \times \vec{S}_1 \cdot \vec{v}_1 \hat{n} \cdot \vec{v}_2 \log\left(\frac{r}{R_\theta}\right) \hat{n} \cdot \vec{v}_1 - \frac{1648 \hat{n} \times \vec{S}_1 \cdot \vec{v}_1 \vec{v}_1 \cdot \vec{v}_1}{1225} + \frac{96}{25} \hat{n} \times \vec{S}_1 \cdot \vec{v}_1 \vec{v}_1 \cdot \vec{v}_2 + \right. \\ \left. \frac{96}{35} \hat{n} \times \vec{S}_1 \cdot \vec{v}_1 \vec{v}_1 \cdot \vec{v}_1 \log\left(\frac{r}{R_\theta}\right) - \frac{24}{5} \hat{n} \times \vec{S}_1 \cdot \vec{v}_1 \vec{v}_1 \cdot \vec{v}_2 \log\left(\frac{r}{R_\theta}\right) + \frac{1}{\epsilon_d} \left( \frac{32}{7} \hat{n} \times \vec{S}_1 \cdot \vec{v}_1 (\hat{n} \cdot \vec{v}_1)^2 + \right. \right. \\ \left. \left. \frac{8}{5} \vec{S}_1 \times \vec{v}_1 \cdot \vec{v}_2 \hat{n} \cdot \vec{v}_1 - 8 \hat{n} \times \vec{S}_1 \cdot \vec{v}_1 \hat{n} \cdot \vec{v}_2 \hat{n} \cdot \vec{v}_1 - \frac{32}{35} \hat{n} \times \vec{S}_1 \cdot \vec{v}_1 \vec{v}_1 \cdot \vec{v}_1 + \frac{8}{5} \hat{n} \times \vec{S}_1 \cdot \vec{v}_1 \vec{v}_1 \cdot \vec{v}_2 \right) \right) G^3 \Bigg\}$$

{DiagSet[3, 1, 71],

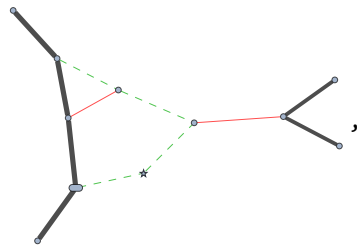

$$\frac{m_1^2 m_2 \left( 8 \log\left(\frac{r}{R_\theta}\right) \hat{n} \times \vec{S}_1 \cdot \vec{a}_1 - \frac{8 \hat{n} \times \vec{S}_1 \cdot \vec{a}_1}{3 \epsilon_d} + \frac{8}{3} \hat{n} \times \vec{S}_1 \cdot \vec{a}_1 \right) G^3}{r^2} + \frac{1}{r^3} m_1^2 m_2 \left( -8 \log\left(\frac{r}{R_\theta}\right) \vec{S}_1 \times \vec{v}_1 \cdot \vec{v}_2 - \frac{8}{3} \vec{S}_1 \times \vec{v}_1 \cdot \vec{v}_2 - \right. \\ \left. \frac{72}{25} \vec{S}_1 \times \vec{v}_1 \cdot \vec{a}_1 + \frac{56}{25} \hat{n} \times \vec{S}_1 \cdot \vec{v}_1 \hat{n} \cdot \vec{a}_1 - \frac{16}{25} \hat{n} \times \vec{S}_1 \cdot \vec{v}_1 \hat{n} \cdot \vec{v}_1 - \frac{8}{5} \hat{n} \times \vec{S}_1 \cdot \vec{a}_1 \hat{n} \cdot \vec{v}_1 + \frac{8}{5} \vec{S}_1 \times \vec{v}_1 \cdot \vec{a}_1 \log\left(\frac{r}{R_\theta}\right) - \right. \\ \left. \frac{24}{5} \hat{n} \times \vec{S}_1 \cdot \vec{v}_1 \hat{n} \cdot \vec{a}_1 \log\left(\frac{r}{R_\theta}\right) - \frac{96}{5} \hat{n} \times \vec{S}_1 \cdot \vec{v}_1 \hat{n} \cdot \vec{v}_1 \log\left(\frac{r}{R_\theta}\right) + 24 \hat{n} \times \vec{S}_1 \cdot \vec{v}_1 \hat{n} \cdot \vec{v}_2 \log\left(\frac{r}{R_\theta}\right) + \frac{1}{\epsilon_d} \right. \\ \left. \left( \frac{8}{3} \vec{S}_1 \times \vec{v}_1 \cdot \vec{v}_2 - \frac{8}{15} \vec{S}_1 \times \vec{v}_1 \cdot \vec{a}_1 + \frac{8}{5} \hat{n} \times \vec{S}_1 \cdot \vec{v}_1 \hat{n} \cdot \vec{a}_1 + \frac{32}{5} \hat{n} \times \vec{S}_1 \cdot \vec{v}_1 \hat{n} \cdot \vec{v}_1 - 8 \hat{n} \times \vec{S}_1 \cdot \vec{v}_1 \hat{n} \cdot \vec{v}_2 \right) \right) G^3 + \frac{1}{r^4} \\ m_1^2 m_2 \left( -\frac{240}{49} \hat{n} \times \vec{S}_1 \cdot \vec{v}_1 (\hat{n} \cdot \vec{v}_1)^2 + \frac{96}{7} \hat{n} \times \vec{S}_1 \cdot \vec{v}_1 \log\left(\frac{r}{R_\theta}\right) (\hat{n} \cdot \vec{v}_1)^2 - \frac{16}{25} \vec{S}_1 \times \vec{v}_1 \cdot \vec{v}_2 \hat{n} \cdot \vec{v}_1 + 8 \hat{n} \times \vec{S}_1 \cdot \vec{v}_1 \hat{n} \cdot \vec{v}_2 \hat{n} \cdot \vec{v}_1 + \right. \\ \left. \frac{24}{5} \vec{S}_1 \times \vec{v}_1 \cdot \vec{v}_2 \log\left(\frac{r}{R_\theta}\right) \hat{n} \cdot \vec{v}_1 - 24 \hat{n} \times \vec{S}_1 \cdot \vec{v}_1 \hat{n} \cdot \vec{v}_2 \log\left(\frac{r}{R_\theta}\right) \hat{n} \cdot \vec{v}_1 - \frac{592 \hat{n} \times \vec{S}_1 \cdot \vec{v}_1 \vec{v}_1 \cdot \vec{v}_1}{1225} - \frac{16}{25} \hat{n} \times \vec{S}_1 \cdot \vec{v}_1 \vec{v}_1 \cdot \vec{v}_2 - \right. \\ \left. \frac{96}{35} \hat{n} \times \vec{S}_1 \cdot \vec{v}_1 \vec{v}_1 \cdot \vec{v}_1 \log\left(\frac{r}{R_\theta}\right) + \frac{24}{5} \hat{n} \times \vec{S}_1 \cdot \vec{v}_1 \vec{v}_1 \cdot \vec{v}_2 \log\left(\frac{r}{R_\theta}\right) + \frac{1}{\epsilon_d} \left( -\frac{32}{7} \hat{n} \times \vec{S}_1 \cdot \vec{v}_1 (\hat{n} \cdot \vec{v}_1)^2 - \right. \right. \\ \left. \left. \frac{8}{5} \vec{S}_1 \times \vec{v}_1 \cdot \vec{v}_2 \hat{n} \cdot \vec{v}_1 + 8 \hat{n} \times \vec{S}_1 \cdot \vec{v}_1 \hat{n} \cdot \vec{v}_2 \hat{n} \cdot \vec{v}_1 + \frac{32}{35} \hat{n} \times \vec{S}_1 \cdot \vec{v}_1 \vec{v}_1 \cdot \vec{v}_1 - \frac{8}{5} \hat{n} \times \vec{S}_1 \cdot \vec{v}_1 \vec{v}_1 \cdot \vec{v}_2 \right) \right) G^3 \Bigg\}$$

{DiagSet[3, 1, 72],

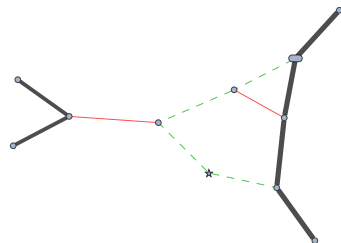

$$, \frac{m_1^2 m_2 \left( -4 \log\left(\frac{r}{R_\theta}\right) \hat{n} \times \vec{S}_1 \cdot \vec{a}_1 + \frac{4 \hat{n} \times \vec{S}_1 \cdot \vec{a}_1}{3 \epsilon_d} + 2 \hat{n} \times \vec{S}_1 \cdot \vec{a}_1 \right) G^3}{r^2} +$$

$$\frac{1}{r^3} m_1^2 m_2 \left( 4 \log\left(\frac{r}{R_\theta}\right) \vec{S}_1 \times \vec{a}_1 \cdot \vec{v}_2 - 2 \vec{S}_1 \times \vec{a}_1 \cdot \vec{v}_2 - \frac{184}{75} \vec{S}_1 \times \vec{v}_1 \cdot \vec{a}_1 + \frac{56}{25} \hat{n} \times \vec{S}_1 \cdot \vec{v}_1 \hat{n} \cdot \vec{a}_1 - \frac{58}{25} \hat{n} \times \vec{S}_1 \cdot \vec{v}_1 \hat{n} \cdot \vec{v}_1 - \right. \\ \left. \frac{248}{25} \hat{n} \times \vec{S}_1 \cdot \vec{a}_1 \hat{n} \cdot \vec{v}_1 + 10 \hat{n} \times \vec{S}_1 \cdot \vec{a}_1 \hat{n} \cdot \vec{v}_2 + \frac{32}{5} \vec{S}_1 \times \vec{v}_1 \cdot \vec{a}_1 \log\left(\frac{r}{R_\theta}\right) - \frac{24}{5} \hat{n} \times \vec{S}_1 \cdot \vec{v}_1 \hat{n} \cdot \vec{a}_1 \log\left(\frac{r}{R_\theta}\right) + \right. \\ \left. \frac{12}{5} \hat{n} \times \vec{S}_1 \cdot \vec{v}_1 \hat{n} \cdot \vec{v}_1 \log\left(\frac{r}{R_\theta}\right) + \frac{72}{5} \hat{n} \times \vec{S}_1 \cdot \vec{a}_1 \hat{n} \cdot \vec{v}_1 \log\left(\frac{r}{R_\theta}\right) - 12 \hat{n} \times \vec{S}_1 \cdot \vec{a}_1 \hat{n} \cdot \vec{v}_2 \log\left(\frac{r}{R_\theta}\right) + \frac{1}{\epsilon_d} \left( -\frac{4}{3} \vec{S}_1 \times \vec{a}_1 \cdot \vec{v}_2 - \right. \right. \\ \left. \left. \frac{4}{3} \vec{S}_1 \times \vec{a}_1 \cdot \vec{v}_2 - \frac{4}{3} \vec{S}_1 \times \vec{a}_1 \cdot \vec{v}_2 \right) \right) G^3 \Bigg\}$$

$$\begin{aligned}
& \left. \frac{32}{15} \vec{S}_1 \times \vec{v}_1 \cdot \vec{a}_1 + \frac{8}{5} \hat{n} \times \vec{S}_1 \cdot \vec{v}_1 \hat{n} \cdot \vec{a}_1 - \frac{4}{5} \hat{n} \times \vec{S}_1 \cdot \vec{v}_1 \hat{n} \cdot \vec{v}_1 - \frac{24}{5} \hat{n} \times \vec{S}_1 \cdot \vec{a}_1 \hat{n} \cdot \vec{v}_1 + 4 \hat{n} \times \vec{S}_1 \cdot \vec{a}_1 \hat{n} \cdot \vec{v}_2 \right) \left( G^3 + \frac{1}{r^4} \right. \\
& m_1^2 m_2 \left( \frac{400}{49} \hat{n} \times \vec{S}_1 \cdot \vec{v}_1 (\hat{n} \cdot \vec{v}_1)^2 - \frac{48}{7} \hat{n} \times \vec{S}_1 \cdot \vec{v}_1 \log \left( \frac{r}{R_\theta} \right) (\hat{n} \cdot \vec{v}_1)^2 + \frac{58}{25} \vec{S}_1 \times \vec{v}_1 \cdot \vec{v}_2 \hat{n} \cdot \vec{v}_1 - 14 \hat{n} \times \vec{S}_1 \cdot \vec{v}_1 \hat{n} \cdot \vec{v}_2 \hat{n} \cdot \vec{v}_1 - \right. \\
& \frac{12}{5} \vec{S}_1 \times \vec{v}_1 \cdot \vec{v}_2 \log \left( \frac{r}{R_\theta} \right) \hat{n} \cdot \vec{v}_1 + 12 \hat{n} \times \vec{S}_1 \cdot \vec{v}_1 \hat{n} \cdot \vec{v}_2 \log \left( \frac{r}{R_\theta} \right) \hat{n} \cdot \vec{v}_1 - \frac{1104 \hat{n} \times \vec{S}_1 \cdot \vec{v}_1 \vec{v}_1 \cdot \vec{v}_1}{1225} + \frac{58}{25} \hat{n} \times \vec{S}_1 \cdot \vec{v}_1 \vec{v}_1 \cdot \vec{v}_2 + \\
& \frac{48}{35} \hat{n} \times \vec{S}_1 \cdot \vec{v}_1 \vec{v}_1 \cdot \vec{v}_1 \log \left( \frac{r}{R_\theta} \right) - \frac{12}{5} \hat{n} \times \vec{S}_1 \cdot \vec{v}_1 \vec{v}_1 \cdot \vec{v}_2 \log \left( \frac{r}{R_\theta} \right) + \frac{1}{\epsilon_d} \left( \frac{16}{7} \hat{n} \times \vec{S}_1 \cdot \vec{v}_1 (\hat{n} \cdot \vec{v}_1)^2 + \right. \\
& \left. \left. \frac{4}{5} \vec{S}_1 \times \vec{v}_1 \cdot \vec{v}_2 \hat{n} \cdot \vec{v}_1 - 4 \hat{n} \times \vec{S}_1 \cdot \vec{v}_1 \hat{n} \cdot \vec{v}_2 \hat{n} \cdot \vec{v}_1 - \frac{16}{35} \hat{n} \times \vec{S}_1 \cdot \vec{v}_1 \vec{v}_1 \cdot \vec{v}_1 + \frac{4}{5} \hat{n} \times \vec{S}_1 \cdot \vec{v}_1 \vec{v}_1 \cdot \vec{v}_2 \right) \right) \left( G^3 \right) \}
\end{aligned}$$

{DiagSet[3, 1, 73],

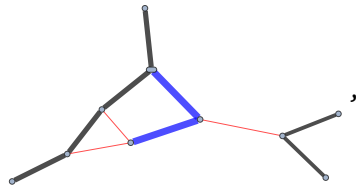

$$\begin{aligned}
& \frac{1}{r^3} G^3 m_1^2 m_2 \left( \frac{-\frac{1}{5} \hat{n} \cdot \vec{a}_1 \hat{n} \times \vec{S}_1 \cdot \vec{v}_1 - \frac{2}{5} \hat{n} \cdot \vec{v}_1 \hat{n} \times \vec{S}_1 \cdot \vec{a}_1 - \frac{1}{15} \vec{S}_1 \times \vec{v}_1 \cdot \vec{a}_1 - \frac{3}{5} \hat{n} \cdot \vec{v}_1 \hat{n} \times \vec{S}_1 \cdot \vec{v}_1}{\epsilon_d} + \right. \\
& \frac{3}{5} \log \left( \frac{r}{R_\theta} \right) \hat{n} \cdot \vec{a}_1 \hat{n} \times \vec{S}_1 \cdot \vec{v}_1 + \frac{6}{5} \log \left( \frac{r}{R_\theta} \right) \hat{n} \cdot \vec{v}_1 \hat{n} \times \vec{S}_1 \cdot \vec{a}_1 - \frac{17}{25} \hat{n} \cdot \vec{a}_1 \hat{n} \times \vec{S}_1 \cdot \vec{v}_1 - \frac{24}{25} \hat{n} \cdot \vec{v}_1 \hat{n} \times \vec{S}_1 \cdot \vec{a}_1 + \\
& \left. \frac{1}{5} \log \left( \frac{r}{R_\theta} \right) \vec{S}_1 \times \vec{v}_1 \cdot \vec{a}_1 + \frac{1}{25} \vec{S}_1 \times \vec{v}_1 \cdot \vec{a}_1 + \frac{9}{5} \log \left( \frac{r}{R_\theta} \right) \hat{n} \cdot \vec{v}_1 \hat{n} \times \vec{S}_1 \cdot \vec{v}_1 - \frac{41}{25} \hat{n} \cdot \vec{v}_1 \hat{n} \times \vec{S}_1 \cdot \vec{v}_1 \right) + \\
& \frac{1}{r^4} G^3 m_1^2 m_2 \left( \frac{\frac{5}{7} (\hat{n} \cdot \vec{v}_1)^2 \hat{n} \times \vec{S}_1 \cdot \vec{v}_1 - \frac{1}{7} \vec{v}_1 \cdot \vec{v}_1 \hat{n} \times \vec{S}_1 \cdot \vec{v}_1}{\epsilon_d} - \frac{15}{7} \log \left( \frac{r}{R_\theta} \right) (\hat{n} \cdot \vec{v}_1)^2 \hat{n} \times \vec{S}_1 \cdot \vec{v}_1 + \right. \\
& \left. \frac{3}{7} \log \left( \frac{r}{R_\theta} \right) \vec{v}_1 \cdot \vec{v}_1 \hat{n} \times \vec{S}_1 \cdot \vec{v}_1 + \frac{90}{49} (\hat{n} \cdot \vec{v}_1)^2 \hat{n} \times \vec{S}_1 \cdot \vec{v}_1 + \frac{3}{49} \vec{v}_1 \cdot \vec{v}_1 \hat{n} \times \vec{S}_1 \cdot \vec{v}_1 \right) \}
\end{aligned}$$

{DiagSet[3, 1, 74],

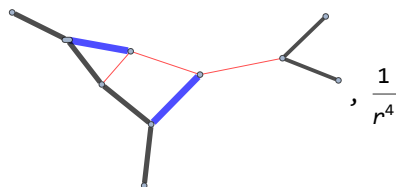

$$\begin{aligned}
& G^3 m_1^2 m_2 \left( \frac{\frac{4}{5} \vec{v}_1 \cdot \vec{v}_1 \hat{n} \times \vec{S}_1 \cdot \vec{v}_1 - 4 (\hat{n} \cdot \vec{v}_1)^2 \hat{n} \times \vec{S}_1 \cdot \vec{v}_1}{\epsilon_d} + 12 \log \left( \frac{r}{R_\theta} \right) (\hat{n} \cdot \vec{v}_1)^2 \hat{n} \times \vec{S}_1 \cdot \vec{v}_1 - \right. \\
& \left. \frac{12}{5} \log \left( \frac{r}{R_\theta} \right) \vec{v}_1 \cdot \vec{v}_1 \hat{n} \times \vec{S}_1 \cdot \vec{v}_1 - 6 (\hat{n} \cdot \vec{v}_1)^2 \hat{n} \times \vec{S}_1 \cdot \vec{v}_1 + \frac{18}{25} \vec{v}_1 \cdot \vec{v}_1 \hat{n} \times \vec{S}_1 \cdot \vec{v}_1 \right) \}
\end{aligned}$$

{DiagSet[3, 1, 75],

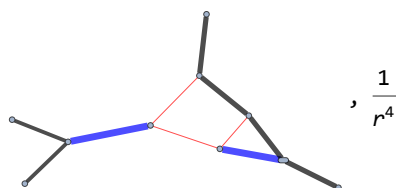



$$G^3 m_1^2 m_2 \left( \frac{\frac{4}{7} (\hat{n} \cdot \vec{v}_2)^2 \hat{n} \times \vec{S}_1 \cdot \vec{v}_1 - \frac{8}{35} \hat{n} \cdot \vec{v}_2 \vec{S}_1 \times \vec{v}_1 \cdot \vec{v}_2 - \frac{4}{35} \vec{v}_2 \cdot \vec{v}_2 \hat{n} \times \vec{S}_1 \cdot \vec{v}_1}{\epsilon_d} - \frac{12}{7} \log\left(\frac{r}{R_\theta}\right) (\hat{n} \cdot \vec{v}_2)^2 \hat{n} \times \vec{S}_1 \cdot \vec{v}_1 + \frac{24}{35} \log\left(\frac{r}{R_\theta}\right) \hat{n} \cdot \vec{v}_2 \vec{S}_1 \times \vec{v}_1 \cdot \vec{v}_2 + \frac{12}{35} \log\left(\frac{r}{R_\theta}\right) \vec{v}_2 \cdot \vec{v}_2 \hat{n} \times \vec{S}_1 \cdot \vec{v}_1 + \frac{58}{49} (\hat{n} \cdot \vec{v}_2)^2 \hat{n} \times \vec{S}_1 \cdot \vec{v}_1 - \frac{377 \hat{n} \cdot \vec{v}_2 \vec{S}_1 \times \vec{v}_1 \cdot \vec{v}_2}{1225} - \frac{66 \vec{v}_2 \cdot \vec{v}_2 \hat{n} \times \vec{S}_1 \cdot \vec{v}_1}{1225} \right)$$

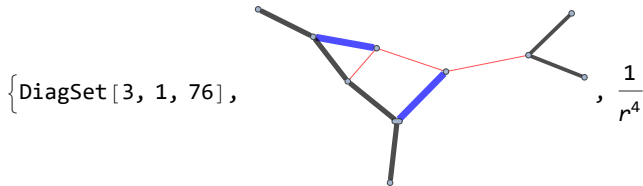

$$G^3 m_1^2 m_2 \left( \frac{\frac{104}{7} (\hat{n} \cdot \vec{v}_1)^2 \hat{n} \times \vec{S}_1 \cdot \vec{v}_1 - \frac{104}{35} \vec{v}_1 \cdot \vec{v}_1 \hat{n} \times \vec{S}_1 \cdot \vec{v}_1}{\epsilon_d} - \frac{312}{7} \log\left(\frac{r}{R_\theta}\right) (\hat{n} \cdot \vec{v}_1)^2 \hat{n} \times \vec{S}_1 \cdot \vec{v}_1 + \frac{312}{35} \log\left(\frac{r}{R_\theta}\right) \vec{v}_1 \cdot \vec{v}_1 \hat{n} \times \vec{S}_1 \cdot \vec{v}_1 + \frac{2572}{49} (\hat{n} \cdot \vec{v}_1)^2 \hat{n} \times \vec{S}_1 \cdot \vec{v}_1 - \frac{11936 \vec{v}_1 \cdot \vec{v}_1 \hat{n} \times \vec{S}_1 \cdot \vec{v}_1}{1225} \right)$$

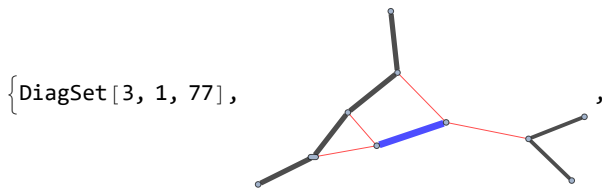

$$\frac{1}{r^3} G^3 m_1^2 m_2 \left( \frac{-\frac{2}{5} \hat{n} \cdot \vec{v}_1 \hat{n} \times \vec{S}_1 \cdot \vec{a}_1 - \frac{2}{15} \vec{S}_1 \times \vec{v}_1 \cdot \vec{a}_1 - \frac{2}{5} \hat{n} \cdot \vec{v}_1 \hat{n} \times \vec{S}_1 \cdot \vec{v}_1}{\epsilon_d} + \frac{6}{5} \log\left(\frac{r}{R_\theta}\right) \hat{n} \cdot \vec{v}_1 \hat{n} \times \vec{S}_1 \cdot \vec{a}_1 - \frac{44}{25} \hat{n} \cdot \vec{v}_1 \hat{n} \times \vec{S}_1 \cdot \vec{a}_1 + \frac{2}{5} \log\left(\frac{r}{R_\theta}\right) \vec{S}_1 \times \vec{v}_1 \cdot \vec{a}_1 + \frac{26}{75} \vec{S}_1 \times \vec{v}_1 \cdot \vec{a}_1 + \frac{6}{5} \log\left(\frac{r}{R_\theta}\right) \hat{n} \cdot \vec{v}_1 \hat{n} \times \vec{S}_1 \cdot \vec{v}_1 - \frac{44}{25} \hat{n} \cdot \vec{v}_1 \hat{n} \times \vec{S}_1 \cdot \vec{v}_1 \right) + \frac{1}{r^4} G^3 m_1^2 m_2 \left( \frac{1}{\epsilon_d} \left( \frac{6}{7} (\hat{n} \cdot \vec{v}_1)^2 \hat{n} \times \vec{S}_1 \cdot \vec{v}_1 + \frac{2}{5} \hat{n} \cdot \vec{v}_1 \vec{S}_1 \times \vec{v}_1 \cdot \vec{v}_2 - 2 \hat{n} \cdot \vec{v}_2 \hat{n} \cdot \vec{v}_1 \hat{n} \times \vec{S}_1 \cdot \vec{v}_1 - \frac{6}{35} \vec{v}_1 \cdot \vec{v}_1 \hat{n} \times \vec{S}_1 \cdot \vec{v}_1 + \frac{2}{5} \vec{v}_1 \cdot \vec{v}_2 \hat{n} \times \vec{S}_1 \cdot \vec{v}_1 \right) - \frac{18}{7} \log\left(\frac{r}{R_\theta}\right) (\hat{n} \cdot \vec{v}_1)^2 \hat{n} \times \vec{S}_1 \cdot \vec{v}_1 - \frac{6}{5} \log\left(\frac{r}{R_\theta}\right) \hat{n} \cdot \vec{v}_1 \vec{S}_1 \times \vec{v}_1 \cdot \vec{v}_2 + 6 \log\left(\frac{r}{R_\theta}\right) \hat{n} \cdot \vec{v}_2 \hat{n} \cdot \vec{v}_1 \hat{n} \times \vec{S}_1 \cdot \vec{v}_1 + \frac{18}{35} \log\left(\frac{r}{R_\theta}\right) \vec{v}_1 \cdot \vec{v}_1 \hat{n} \times \vec{S}_1 \cdot \vec{v}_1 - \frac{6}{5} \log\left(\frac{r}{R_\theta}\right) \vec{v}_1 \cdot \vec{v}_2 \hat{n} \times \vec{S}_1 \cdot \vec{v}_1 + \frac{199}{49} (\hat{n} \cdot \vec{v}_1)^2 \hat{n} \times \vec{S}_1 \cdot \vec{v}_1 + \frac{19}{25} \hat{n} \cdot \vec{v}_1 \vec{S}_1 \times \vec{v}_1 \cdot \vec{v}_2 - 5 \hat{n} \cdot \vec{v}_2 \hat{n} \cdot \vec{v}_1 \hat{n} \times \vec{S}_1 \cdot \vec{v}_1 + \frac{2036 \vec{v}_1 \cdot \vec{v}_1 \hat{n} \times \vec{S}_1 \cdot \vec{v}_1}{1225} + \frac{19}{25} \vec{v}_1 \cdot \vec{v}_2 \hat{n} \times \vec{S}_1 \cdot \vec{v}_1 + \frac{6}{5} \vec{v}_2 \cdot \vec{v}_2 \hat{n} \times \vec{S}_1 \cdot \vec{v}_1 \right) \right)$$

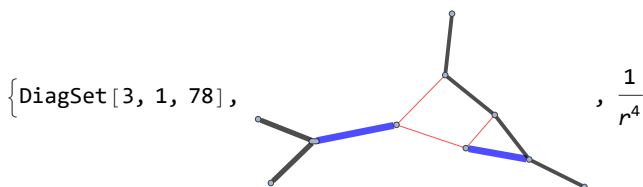

$$G^3 m_2^3 \left( \frac{1}{\epsilon_d} \left( \frac{32}{7} (\hat{n} \cdot \vec{v}_2)^2 \hat{n} \times \vec{S}_1 \cdot \vec{v}_1 - \frac{8}{5} \hat{n} \cdot \vec{v}_2 \vec{S}_1 \times \vec{v}_1 \cdot \vec{v}_2 + \frac{8}{7} \hat{n} \cdot \vec{v}_1 \hat{n} \cdot \vec{v}_2 \hat{n} \times \vec{S}_1 \cdot \vec{v}_2 - \right.$$

$$\begin{aligned} & \frac{8}{35} \vec{v}_1 \cdot \vec{v}_2 \hat{n} \times \vec{S}_1 \cdot \vec{v}_2 - \frac{32}{35} \vec{v}_2 \cdot \vec{v}_2 \hat{n} \times \vec{S}_1 \cdot \vec{v}_1 \Big) - \frac{96}{7} \log\left(\frac{r}{R_\theta}\right) (\hat{n} \cdot \vec{v}_2)^2 \hat{n} \times \vec{S}_1 \cdot \vec{v}_1 + \\ & \frac{24}{5} \log\left(\frac{r}{R_\theta}\right) \hat{n} \cdot \vec{v}_2 \vec{S}_1 \times \vec{v}_1 \cdot \vec{v}_2 - \frac{24}{7} \log\left(\frac{r}{R_\theta}\right) \hat{n} \cdot \vec{v}_1 \hat{n} \cdot \vec{v}_2 \hat{n} \times \vec{S}_1 \cdot \vec{v}_2 + \frac{24}{35} \log\left(\frac{r}{R_\theta}\right) \vec{v}_1 \cdot \vec{v}_2 \hat{n} \times \vec{S}_1 \cdot \vec{v}_2 + \\ & \frac{96}{35} \log\left(\frac{r}{R_\theta}\right) \vec{v}_2 \cdot \vec{v}_2 \hat{n} \times \vec{S}_1 \cdot \vec{v}_1 + \frac{800}{49} (\hat{n} \cdot \vec{v}_2)^2 \hat{n} \times \vec{S}_1 \cdot \vec{v}_1 - \frac{116}{25} \hat{n} \cdot \vec{v}_2 \vec{S}_1 \times \vec{v}_1 \cdot \vec{v}_2 + \\ & \left. \frac{228}{49} \hat{n} \cdot \vec{v}_1 \hat{n} \cdot \vec{v}_2 \hat{n} \times \vec{S}_1 \cdot \vec{v}_2 - \frac{2652 \vec{v}_1 \cdot \vec{v}_2 \hat{n} \times \vec{S}_1 \cdot \vec{v}_2}{1225} - \frac{4168 \vec{v}_2 \cdot \vec{v}_2 \hat{n} \times \vec{S}_1 \cdot \vec{v}_1}{1225} \right\} \end{aligned}$$

$\{\text{DiagSet}[3, 1, 79],$ 
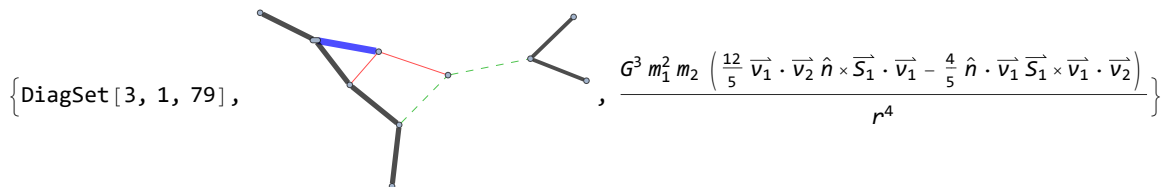
 $, \frac{G^3 m_1^2 m_2 \left( \frac{12}{5} \vec{v}_1 \cdot \vec{v}_2 \hat{n} \times \vec{S}_1 \cdot \vec{v}_1 - \frac{4}{5} \hat{n} \cdot \vec{v}_1 \vec{S}_1 \times \vec{v}_1 \cdot \vec{v}_2 \right)}{r^4} \}$

$\{\text{DiagSet}[3, 1, 80],$ 
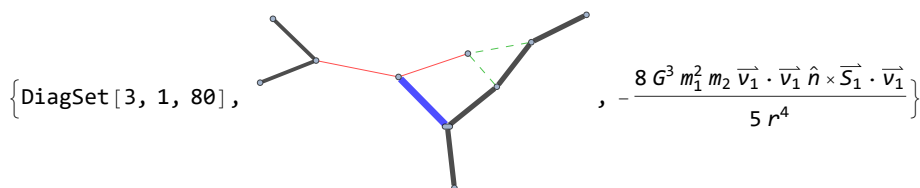
 $, -\frac{8 G^3 m_1^2 m_2 \vec{v}_1 \cdot \vec{v}_1 \hat{n} \times \vec{S}_1 \cdot \vec{v}_1}{5 r^4} \}$

$\{\text{DiagSet}[3, 1, 81],$ 
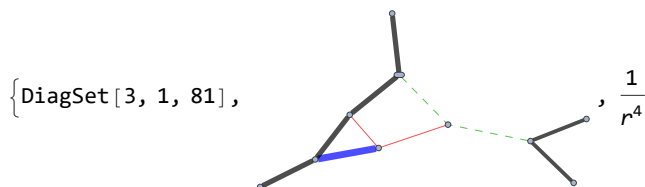
 $, \frac{1}{r^4}$

$$\begin{aligned} & G^3 m_1^2 m_2 \left( \frac{1}{\epsilon_d} \left( -\frac{32}{7} (\hat{n} \cdot \vec{v}_1)^2 \hat{n} \times \vec{S}_1 \cdot \vec{v}_2 - \frac{32}{7} \hat{n} \cdot \vec{v}_1 \vec{S}_1 \times \vec{v}_1 \cdot \vec{v}_2 + \frac{96}{7} \hat{n} \cdot \vec{v}_2 \hat{n} \cdot \vec{v}_1 \hat{n} \times \vec{S}_1 \cdot \vec{v}_1 + \right. \right. \\ & \frac{32}{35} \vec{v}_1 \cdot \vec{v}_1 \hat{n} \times \vec{S}_1 \cdot \vec{v}_2 - \frac{96}{35} \vec{v}_1 \cdot \vec{v}_2 \hat{n} \times \vec{S}_1 \cdot \vec{v}_1 \Big) + \frac{96}{7} \log\left(\frac{r}{R_\theta}\right) (\hat{n} \cdot \vec{v}_1)^2 \hat{n} \times \vec{S}_1 \cdot \vec{v}_2 + \\ & \frac{96}{7} \log\left(\frac{r}{R_\theta}\right) \hat{n} \cdot \vec{v}_1 \vec{S}_1 \times \vec{v}_1 \cdot \vec{v}_2 - \frac{288}{7} \log\left(\frac{r}{R_\theta}\right) \hat{n} \cdot \vec{v}_2 \hat{n} \cdot \vec{v}_1 \hat{n} \times \vec{S}_1 \cdot \vec{v}_1 - \frac{96}{35} \log\left(\frac{r}{R_\theta}\right) \vec{v}_1 \cdot \vec{v}_1 \hat{n} \times \vec{S}_1 \cdot \vec{v}_2 + \\ & \frac{288}{35} \log\left(\frac{r}{R_\theta}\right) \vec{v}_1 \cdot \vec{v}_2 \hat{n} \times \vec{S}_1 \cdot \vec{v}_1 - \frac{128}{49} (\hat{n} \cdot \vec{v}_1)^2 \hat{n} \times \vec{S}_1 \cdot \vec{v}_2 - \frac{3552}{245} \hat{n} \cdot \vec{v}_1 \vec{S}_1 \times \vec{v}_1 \cdot \vec{v}_2 + \\ & \left. \frac{1952}{49} \hat{n} \cdot \vec{v}_2 \hat{n} \cdot \vec{v}_1 \hat{n} \times \vec{S}_1 \cdot \vec{v}_1 - \frac{5072 \vec{v}_1 \cdot \vec{v}_1 \hat{n} \times \vec{S}_1 \cdot \vec{v}_2}{1225} - \frac{4384 \vec{v}_1 \cdot \vec{v}_2 \hat{n} \times \vec{S}_1 \cdot \vec{v}_1}{1225} \right\} \end{aligned}$$

$\{\text{DiagSet}[3, 1, 82],$ 
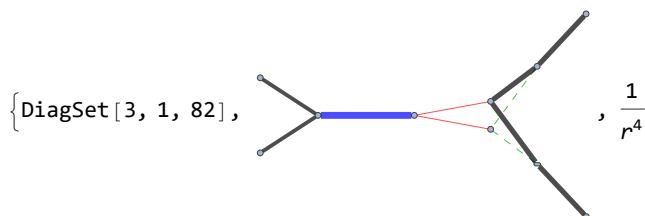
 $, \frac{1}{r^4}$

$$\begin{aligned} & G^3 m_1^2 m_2 \left( \frac{-\frac{16}{7} (\hat{n} \cdot \vec{v}_2)^2 \hat{n} \times \vec{S}_1 \cdot \vec{v}_1 + \frac{32}{35} \hat{n} \cdot \vec{v}_2 \vec{S}_1 \times \vec{v}_1 \cdot \vec{v}_2 + \frac{16}{35} \vec{v}_2 \cdot \vec{v}_2 \hat{n} \times \vec{S}_1 \cdot \vec{v}_1}{\epsilon_d} + \right. \\ & \frac{48}{7} \log\left(\frac{r}{R_\theta}\right) (\hat{n} \cdot \vec{v}_2)^2 \hat{n} \times \vec{S}_1 \cdot \vec{v}_1 - \frac{96}{35} \log\left(\frac{r}{R_\theta}\right) \hat{n} \cdot \vec{v}_2 \vec{S}_1 \times \vec{v}_1 \cdot \vec{v}_2 - \frac{48}{35} \log\left(\frac{r}{R_\theta}\right) \vec{v}_2 \cdot \vec{v}_2 \hat{n} \times \vec{S}_1 \cdot \vec{v}_1 - \end{aligned}$$

$$\frac{288}{49} (\hat{n} \cdot \vec{v}_2)^2 \hat{n} \times \vec{S}_1 \cdot \vec{v}_1 + \frac{2068 \hat{n} \cdot \vec{v}_2 \vec{S}_1 \times \vec{v}_1 \cdot \vec{v}_2}{1225} + \frac{544 \vec{v}_2 \cdot \vec{v}_2 \hat{n} \times \vec{S}_1 \cdot \vec{v}_1}{1225} \Bigg\}$$

{DiagSet[3, 1, 83], 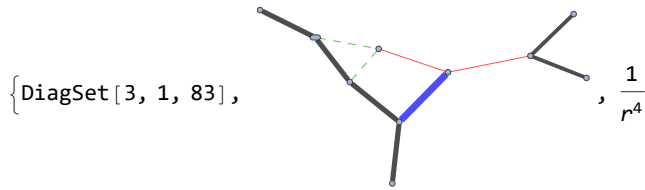 ,  $\frac{1}{r^4}$ }

$$G^3 m_1^2 m_2 \left( \frac{16 (\hat{n} \cdot \vec{v}_1)^2 \hat{n} \times \vec{S}_1 \cdot \vec{v}_1 - \frac{16}{5} \vec{v}_1 \cdot \vec{v}_1 \hat{n} \times \vec{S}_1 \cdot \vec{v}_1}{\epsilon_d} - 48 \log\left(\frac{r}{R_\theta}\right) (\hat{n} \cdot \vec{v}_1)^2 \hat{n} \times \vec{S}_1 \cdot \vec{v}_1 + \right.$$

$$\left. \frac{48}{5} \log\left(\frac{r}{R_\theta}\right) \vec{v}_1 \cdot \vec{v}_1 \hat{n} \times \vec{S}_1 \cdot \vec{v}_1 + 32 (\hat{n} \cdot \vec{v}_1)^2 \hat{n} \times \vec{S}_1 \cdot \vec{v}_1 - \frac{112}{25} \vec{v}_1 \cdot \vec{v}_1 \hat{n} \times \vec{S}_1 \cdot \vec{v}_1 \right\}$$

{DiagSet[3, 1, 84], 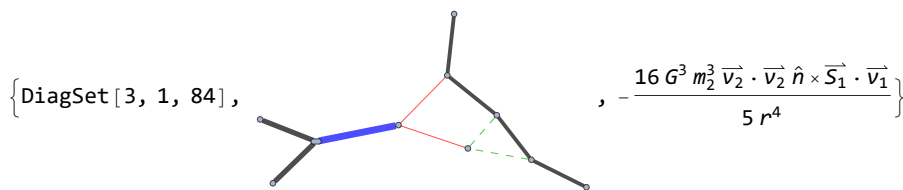 ,  $-\frac{16 G^3 m_2^3 \vec{v}_2 \cdot \vec{v}_2 \hat{n} \times \vec{S}_1 \cdot \vec{v}_1}{5 r^4}$ }

{DiagSet[3, 1, 85], 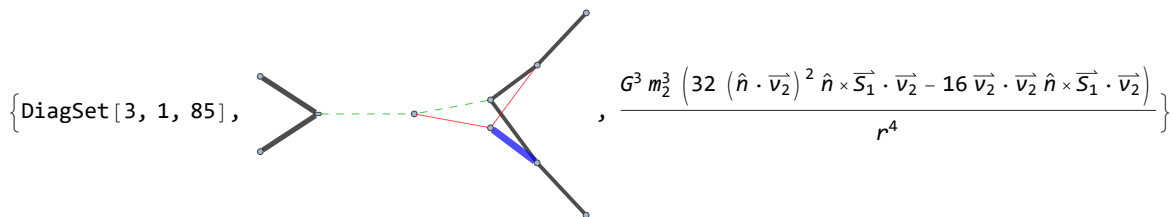 ,  $\frac{G^3 m_2^3 \left( 32 (\hat{n} \cdot \vec{v}_2)^2 \hat{n} \times \vec{S}_1 \cdot \vec{v}_2 - 16 \vec{v}_2 \cdot \vec{v}_2 \hat{n} \times \vec{S}_1 \cdot \vec{v}_2 \right)}{r^4}$ }

{DiagSet[3, 1, 86], 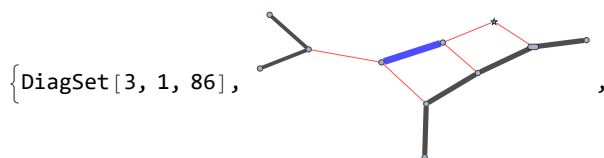 ,

$$\frac{1}{r^3} m_1^2 m_2 \left( -2 \log\left(\frac{r}{R_\theta}\right) \vec{S}_1 \times \vec{v}_1 \cdot \vec{v}_2 + \frac{13}{9} \vec{S}_1 \times \vec{v}_1 \cdot \vec{v}_2 + \frac{13}{9} \vec{S}_1 \times \vec{a}_1 \cdot \vec{v}_2 + \frac{412}{225} \vec{S}_1 \times \vec{v}_1 \cdot \vec{a}_1 + \frac{472}{75} \hat{n} \times \vec{S}_1 \cdot \vec{v}_1 \hat{n} \cdot \vec{v}_1 + \right.$$

$$\frac{472}{75} \hat{n} \times \vec{S}_1 \cdot \vec{a}_1 \hat{n} \cdot \vec{v}_1 - \frac{19}{3} \hat{n} \times \vec{S}_1 \cdot \vec{v}_1 \hat{n} \cdot \vec{v}_2 - \frac{19}{3} \hat{n} \times \vec{S}_1 \cdot \vec{a}_1 \hat{n} \cdot \vec{v}_2 - 2 \vec{S}_1 \times \vec{a}_1 \cdot \vec{v}_2 \log\left(\frac{r}{R_\theta}\right) -$$

$$\frac{12}{5} \vec{S}_1 \times \vec{v}_1 \cdot \vec{a}_1 \log\left(\frac{r}{R_\theta}\right) - \frac{36}{5} \hat{n} \times \vec{S}_1 \cdot \vec{v}_1 \hat{n} \cdot \vec{v}_1 \log\left(\frac{r}{R_\theta}\right) - \frac{36}{5} \hat{n} \times \vec{S}_1 \cdot \vec{a}_1 \hat{n} \cdot \vec{v}_1 \log\left(\frac{r}{R_\theta}\right) +$$

$$6 \hat{n} \times \vec{S}_1 \cdot \vec{v}_1 \hat{n} \cdot \vec{v}_2 \log\left(\frac{r}{R_\theta}\right) + 6 \hat{n} \times \vec{S}_1 \cdot \vec{a}_1 \hat{n} \cdot \vec{v}_2 \log\left(\frac{r}{R_\theta}\right) + \frac{1}{\epsilon_d} \left( \frac{2}{3} \vec{S}_1 \times \vec{v}_1 \cdot \vec{v}_2 + \frac{2}{3} \vec{S}_1 \times \vec{a}_1 \cdot \vec{v}_2 + \right.$$

$$\left. \frac{4}{5} \vec{S}_1 \times \vec{v}_1 \cdot \vec{a}_1 + \frac{12}{5} \hat{n} \times \vec{S}_1 \cdot \vec{v}_1 \hat{n} \cdot \vec{v}_1 + \frac{12}{5} \hat{n} \times \vec{S}_1 \cdot \vec{a}_1 \hat{n} \cdot \vec{v}_1 - 2 \hat{n} \times \vec{S}_1 \cdot \vec{v}_1 \hat{n} \cdot \vec{v}_2 - 2 \hat{n} \times \vec{S}_1 \cdot \vec{a}_1 \hat{n} \cdot \vec{v}_2 \right) \Bigg) G^3 +$$

$$\frac{1}{r^4} m_1^2 m_2 \left( -\frac{44}{147} \hat{n} \times \vec{S}_1 \cdot \vec{v}_1 (\hat{n} \cdot \vec{v}_1)^2 - \frac{24}{7} \hat{n} \times \vec{S}_1 \cdot \vec{v}_1 \log\left(\frac{r}{R_\theta}\right) (\hat{n} \cdot \vec{v}_1)^2 - \frac{1}{25} \vec{S}_1 \times \vec{v}_1 \cdot \vec{v}_2 \hat{n} \cdot \vec{v}_1 - \right.$$

$$\hat{n} \times \vec{S}_1 \cdot \vec{v}_1 \hat{n} \cdot \vec{v}_2 \hat{n} \cdot \vec{v}_1 - \frac{6}{5} \vec{S}_1 \times \vec{v}_1 \cdot \vec{v}_2 \log\left(\frac{r}{R_\theta}\right) \hat{n} \cdot \vec{v}_1 + 6 \hat{n} \times \vec{S}_1 \cdot \vec{v}_1 \hat{n} \cdot \vec{v}_2 \log\left(\frac{r}{R_\theta}\right) \hat{n} \cdot \vec{v}_1 + \frac{1564 \hat{n} \times \vec{S}_1 \cdot \vec{v}_1 \vec{v}_1 \cdot \vec{v}_1}{3675} -$$

$$\frac{1}{25} \hat{n} \times \vec{S}_1 \cdot \vec{v}_1 \vec{v}_1 \cdot \vec{v}_2 + \frac{24}{35} \hat{n} \times \vec{S}_1 \cdot \vec{v}_1 \vec{v}_1 \cdot \vec{v}_1 \log\left(\frac{r}{R_\theta}\right) - \frac{6}{5} \hat{n} \times \vec{S}_1 \cdot \vec{v}_1 \vec{v}_1 \cdot \vec{v}_2 \log\left(\frac{r}{R_\theta}\right) + \frac{1}{\epsilon_d} \left( \frac{8}{7} \hat{n} \times \vec{S}_1 \cdot \vec{v}_1 (\hat{n} \cdot \vec{v}_1)^2 + \right.$$

$$\left. \frac{2}{5} \vec{S}_1 \times \vec{v}_1 \cdot \vec{v}_2 \hat{n} \cdot \vec{v}_1 - 2 \hat{n} \times \vec{S}_1 \cdot \vec{v}_1 \hat{n} \cdot \vec{v}_2 \hat{n} \cdot \vec{v}_1 - \frac{8}{35} \hat{n} \times \vec{S}_1 \cdot \vec{v}_1 \vec{v}_1 \cdot \vec{v}_1 + \frac{2}{5} \hat{n} \times \vec{S}_1 \cdot \vec{v}_1 \vec{v}_1 \cdot \vec{v}_2 \right) G^3 \}$$

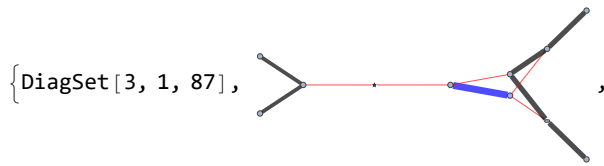

$$\frac{1}{r^3} G^3 m_1^2 m_2 \left( \frac{-\frac{2}{5} \hat{n} \cdot \vec{v}_2 \hat{n} \times \vec{S}_1 \cdot \vec{a}_1 + \frac{2}{15} \vec{S}_1 \times \vec{a}_1 \cdot \vec{v}_2 - \frac{2}{5} \hat{n} \cdot \vec{v}_2 \hat{n} \times \vec{S}_1 \cdot \vec{v}_1 + \frac{2}{15} \vec{S}_1 \times \vec{v}_1 \cdot \vec{v}_2}{\epsilon_d} + \right.$$

$$\frac{6}{5} \log\left(\frac{r}{R_\theta}\right) \hat{n} \cdot \vec{v}_2 \hat{n} \times \vec{S}_1 \cdot \vec{a}_1 - \frac{39}{25} \hat{n} \cdot \vec{v}_2 \hat{n} \times \vec{S}_1 \cdot \vec{a}_1 - \frac{2}{5} \log\left(\frac{r}{R_\theta}\right) \vec{S}_1 \times \vec{a}_1 \cdot \vec{v}_2 + \frac{29}{75} \vec{S}_1 \times \vec{a}_1 \cdot \vec{v}_2 +$$

$$\frac{6}{5} \log\left(\frac{r}{R_\theta}\right) \hat{n} \cdot \vec{v}_2 \hat{n} \times \vec{S}_1 \cdot \vec{v}_1 - \frac{39}{25} \hat{n} \cdot \vec{v}_2 \hat{n} \times \vec{S}_1 \cdot \vec{v}_1 - \frac{2}{5} \log\left(\frac{r}{R_\theta}\right) \vec{S}_1 \times \vec{v}_1 \cdot \vec{v}_2 + \frac{29}{75} \vec{S}_1 \times \vec{v}_1 \cdot \vec{v}_2 \left. \right) +$$

$$\frac{1}{r^4} G^3 m_1^2 m_2 \left( \frac{-\frac{2}{5} \hat{n} \cdot \vec{v}_1 \vec{S}_1 \times \vec{v}_1 \cdot \vec{v}_2 + 2 \hat{n} \cdot \vec{v}_2 \hat{n} \cdot \vec{v}_1 \hat{n} \times \vec{S}_1 \cdot \vec{v}_1 - \frac{2}{5} \vec{v}_1 \cdot \vec{v}_2 \hat{n} \times \vec{S}_1 \cdot \vec{v}_1}{\epsilon_d} + \right.$$

$$\frac{6}{5} \log\left(\frac{r}{R_\theta}\right) \hat{n} \cdot \vec{v}_1 \vec{S}_1 \times \vec{v}_1 \cdot \vec{v}_2 - 6 \log\left(\frac{r}{R_\theta}\right) \hat{n} \cdot \vec{v}_2 \hat{n} \cdot \vec{v}_1 \hat{n} \times \vec{S}_1 \cdot \vec{v}_1 + \frac{6}{5} \log\left(\frac{r}{R_\theta}\right) \vec{v}_1 \cdot \vec{v}_2 \hat{n} \times \vec{S}_1 \cdot \vec{v}_1 -$$

$$\frac{39}{25} \hat{n} \cdot \vec{v}_1 \vec{S}_1 \times \vec{v}_1 \cdot \vec{v}_2 + 9 \hat{n} \cdot \vec{v}_2 \hat{n} \cdot \vec{v}_1 \hat{n} \times \vec{S}_1 \cdot \vec{v}_1 - \frac{39}{25} \vec{v}_1 \cdot \vec{v}_2 \hat{n} \times \vec{S}_1 \cdot \vec{v}_1 \left. \right) \}$$

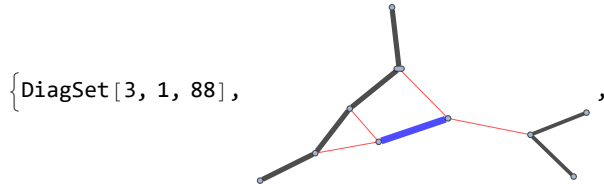

$$\frac{1}{r^3} G^3 m_1^2 m_2 \left( \frac{\hat{n} \cdot \vec{v}_2 \hat{n} \times \vec{S}_1 \cdot \vec{a}_1 - \frac{1}{3} \vec{S}_1 \times \vec{a}_1 \cdot \vec{v}_2 + \hat{n} \cdot \vec{v}_2 \hat{n} \times \vec{S}_1 \cdot \vec{v}_1 - \frac{1}{3} \vec{S}_1 \times \vec{v}_1 \cdot \vec{v}_2}{\epsilon_d} - \right.$$

$$3 \log\left(\frac{r}{R_\theta}\right) \hat{n} \cdot \vec{v}_2 \hat{n} \times \vec{S}_1 \cdot \vec{a}_1 + \frac{3}{2} \hat{n} \cdot \vec{v}_2 \hat{n} \times \vec{S}_1 \cdot \vec{a}_1 + \log\left(\frac{r}{R_\theta}\right) \vec{S}_1 \times \vec{a}_1 \cdot \vec{v}_2 - \frac{1}{6} \vec{S}_1 \times \vec{a}_1 \cdot \vec{v}_2 + \frac{2}{3} \vec{S}_1 \times \vec{v}_1 \cdot \vec{a}_1 -$$

$$3 \log\left(\frac{r}{R_\theta}\right) \hat{n} \cdot \vec{v}_2 \hat{n} \times \vec{S}_1 \cdot \vec{v}_1 + \frac{3}{2} \hat{n} \cdot \vec{v}_2 \hat{n} \times \vec{S}_1 \cdot \vec{v}_1 + \log\left(\frac{r}{R_\theta}\right) \vec{S}_1 \times \vec{v}_1 \cdot \vec{v}_2 - \frac{1}{6} \vec{S}_1 \times \vec{v}_1 \cdot \vec{v}_2 \left. \right) + \frac{1}{r^4} G^3 m_1^2 m_2 \left( \frac{1}{\epsilon_d} \right.$$

$$\left( \frac{1}{7} (\hat{n} \cdot \vec{v}_1)^2 \hat{n} \times \vec{S}_1 \cdot \vec{v}_1 + \frac{3}{5} \hat{n} \cdot \vec{v}_1 \vec{S}_1 \times \vec{v}_1 \cdot \vec{v}_2 - 3 \hat{n} \cdot \vec{v}_2 \hat{n} \cdot \vec{v}_1 \hat{n} \times \vec{S}_1 \cdot \vec{v}_1 - \frac{1}{35} \vec{v}_1 \cdot \vec{v}_1 \hat{n} \times \vec{S}_1 \cdot \vec{v}_1 + \frac{3}{5} \vec{v}_1 \cdot \vec{v}_2 \hat{n} \times \vec{S}_1 \cdot \vec{v}_1 \right) -$$

$$\frac{3}{7} \log\left(\frac{r}{R_\theta}\right) (\hat{n} \cdot \vec{v}_1)^2 \hat{n} \times \vec{S}_1 \cdot \vec{v}_1 - \frac{9}{5} \log\left(\frac{r}{R_\theta}\right) \hat{n} \cdot \vec{v}_1 \vec{S}_1 \times \vec{v}_1 \cdot \vec{v}_2 + 9 \log\left(\frac{r}{R_\theta}\right) \hat{n} \cdot \vec{v}_2 \hat{n} \cdot \vec{v}_1 \hat{n} \times \vec{S}_1 \cdot \vec{v}_1 +$$

$$\frac{3}{35} \log\left(\frac{r}{R_\theta}\right) \vec{v}_1 \cdot \vec{v}_1 \hat{n} \times \vec{S}_1 \cdot \vec{v}_1 - \frac{9}{5} \log\left(\frac{r}{R_\theta}\right) \vec{v}_1 \cdot \vec{v}_2 \hat{n} \times \vec{S}_1 \cdot \vec{v}_1 + \frac{46}{49} (\hat{n} \cdot \vec{v}_1)^2 \hat{n} \times \vec{S}_1 \cdot \vec{v}_1 + \frac{37}{50} \hat{n} \cdot \vec{v}_1 \vec{S}_1 \times \vec{v}_1 \cdot \vec{v}_2 -$$

$$\frac{11}{2} \hat{n} \cdot \vec{v}_2 \hat{n} \cdot \vec{v}_1 \hat{n} \times \vec{S}_1 \cdot \vec{v}_1 + \frac{4481 \vec{v}_1 \cdot \vec{v}_1 \hat{n} \times \vec{S}_1 \cdot \vec{v}_1}{1225} + \frac{37}{50} \vec{v}_1 \cdot \vec{v}_2 \hat{n} \times \vec{S}_1 \cdot \vec{v}_1 + \frac{9}{5} \vec{v}_2 \cdot \vec{v}_2 \hat{n} \times \vec{S}_1 \cdot \vec{v}_1 \left. \right) \}$$

{DiagSet[3, 1, 89],

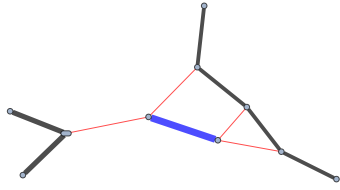

,

$$\frac{1}{r^3} G^3 \left( \log \left( \frac{r}{R_0} \right) \frac{1}{S_1 \times \vec{v}_1 \cdot \vec{v}_2} - \frac{1}{6} \frac{1}{S_1 \times \vec{v}_1 \cdot \vec{v}_2} + \frac{2}{3} \vec{a}_1 \times \vec{S}_1 \cdot \vec{v}_1 + \frac{1}{6} \vec{a}_1 \times \vec{S}_1 \cdot \vec{v}_2 + \right. \\ \left. \frac{3}{2} \hat{n} \times \vec{S}_1 \cdot \vec{v}_1 \hat{n} \cdot \vec{v}_2 - \frac{3}{2} \hat{n} \times \vec{a}_1 \cdot \vec{S}_1 \hat{n} \cdot \vec{v}_2 - \vec{a}_1 \times \vec{S}_1 \cdot \vec{v}_2 \log \left( \frac{r}{R_0} \right) - 3 \hat{n} \times \vec{S}_1 \cdot \vec{v}_1 \hat{n} \cdot \vec{v}_2 \log \left( \frac{r}{R_0} \right) + \right. \\ \left. 3 \hat{n} \times \vec{a}_1 \cdot \vec{S}_1 \hat{n} \cdot \vec{v}_2 \log \left( \frac{r}{R_0} \right) + \frac{-\frac{1}{3} \vec{S}_1 \times \vec{v}_1 \cdot \vec{v}_2 + \frac{1}{3} \vec{a}_1 \times \vec{S}_1 \cdot \vec{v}_2 + \hat{n} \times \vec{S}_1 \cdot \vec{v}_1 \hat{n} \cdot \vec{v}_2 - \hat{n} \times \vec{a}_1 \cdot \vec{S}_1 \hat{n} \cdot \vec{v}_2}{\epsilon_d} \right) m_2^3 + \frac{1}{r^4} \\ G^3 \left( 5 \hat{n} \times \vec{S}_1 \cdot \vec{v}_1 (\hat{n} \cdot \vec{v}_2)^2 - 3 \hat{n} \times \vec{S}_1 \cdot \vec{v}_1 \log \left( \frac{r}{R_0} \right) (\hat{n} \cdot \vec{v}_2)^2 - \frac{44}{25} \vec{S}_1 \times \vec{v}_1 \cdot \vec{v}_2 \hat{n} \cdot \vec{v}_2 - \frac{21}{2} \hat{n} \times \vec{S}_1 \cdot \vec{v}_1 \hat{n} \cdot \vec{v}_1 \hat{n} \cdot \vec{v}_2 + \right. \\ \left. \frac{6}{5} \vec{S}_1 \times \vec{v}_1 \cdot \vec{v}_2 \log \left( \frac{r}{R_0} \right) \hat{n} \cdot \vec{v}_2 + 15 \hat{n} \times \vec{S}_1 \cdot \vec{v}_1 \hat{n} \cdot \vec{v}_1 \log \left( \frac{r}{R_0} \right) \hat{n} \cdot \vec{v}_2 + \frac{3}{2} \vec{S}_1 \times \vec{v}_1 \cdot \vec{v}_2 \hat{n} \cdot \vec{v}_1 + \right. \\ \left. \hat{n} \times \vec{S}_1 \cdot \vec{v}_1 \vec{v}_1 \cdot \vec{v}_1 + \frac{3}{2} \hat{n} \times \vec{S}_1 \cdot \vec{v}_1 \vec{v}_1 \cdot \vec{v}_2 + \frac{183}{25} \hat{n} \times \vec{S}_1 \cdot \vec{v}_1 \vec{v}_2 \cdot \vec{v}_2 - 3 \vec{S}_1 \times \vec{v}_1 \cdot \vec{v}_2 \hat{n} \cdot \vec{v}_1 \log \left( \frac{r}{R_0} \right) - \right. \\ \left. 3 \hat{n} \times \vec{S}_1 \cdot \vec{v}_1 \vec{v}_1 \cdot \vec{v}_2 \log \left( \frac{r}{R_0} \right) + \frac{3}{5} \hat{n} \times \vec{S}_1 \cdot \vec{v}_1 \vec{v}_2 \cdot \vec{v}_2 \log \left( \frac{r}{R_0} \right) + \frac{1}{\epsilon_d} (\hat{n} \times \vec{S}_1 \cdot \vec{v}_1 (\hat{n} \cdot \vec{v}_2)^2 - \frac{2}{5} \vec{S}_1 \times \vec{v}_1 \cdot \vec{v}_2 \hat{n} \cdot \vec{v}_2 - \right. \\ \left. 5 \hat{n} \times \vec{S}_1 \cdot \vec{v}_1 \hat{n} \cdot \vec{v}_1 \hat{n} \cdot \vec{v}_2 + \vec{S}_1 \times \vec{v}_1 \cdot \vec{v}_2 \hat{n} \cdot \vec{v}_1 + \hat{n} \times \vec{S}_1 \cdot \vec{v}_1 \vec{v}_1 \cdot \vec{v}_2 - \frac{1}{5} \hat{n} \times \vec{S}_1 \cdot \vec{v}_1 \vec{v}_2 \cdot \vec{v}_2) \right) m_2^3 \Big\}$$

{DiagSet[3, 1, 90],

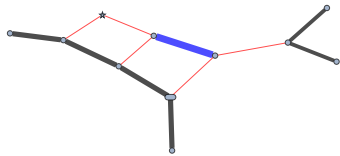

,

$$\frac{1}{r^3} G^3 m_1^2 m_2 \left( \frac{\frac{9}{5} \hat{n} \cdot \vec{v}_1 \hat{n} \times \vec{S}_1 \cdot \vec{a}_1 + \frac{3}{5} \vec{S}_1 \times \vec{v}_1 \cdot \vec{a}_1 + \frac{9}{5} \hat{n} \cdot \vec{v}_1 \hat{n} \times \vec{S}_1 \cdot \vec{v}_1}{\epsilon_d} - \frac{27}{5} \log \left( \frac{r}{R_0} \right) \hat{n} \cdot \vec{v}_1 \hat{n} \times \vec{S}_1 \cdot \vec{a}_1 + \frac{319}{75} \hat{n} \cdot \vec{v}_1 \hat{n} \times \vec{S}_1 \cdot \vec{a}_1 - \right. \\ \left. \frac{9}{5} \log \left( \frac{r}{R_0} \right) \vec{S}_1 \times \vec{v}_1 \cdot \vec{a}_1 + \frac{274}{225} \vec{S}_1 \times \vec{v}_1 \cdot \vec{a}_1 - \frac{27}{5} \log \left( \frac{r}{R_0} \right) \hat{n} \cdot \vec{v}_1 \hat{n} \times \vec{S}_1 \cdot \vec{v}_1 + \frac{319}{75} \hat{n} \cdot \vec{v}_1 \hat{n} \times \vec{S}_1 \cdot \vec{v}_1 \right) + \frac{1}{r^4} \\ G^3 m_1^2 m_2 \left( \frac{1}{\epsilon_d} \left( -\frac{73}{7} (\hat{n} \cdot \vec{v}_1)^2 \hat{n} \times \vec{S}_1 \cdot \vec{v}_1 - \frac{9}{5} \hat{n} \cdot \vec{v}_1 \vec{S}_1 \times \vec{v}_1 \cdot \vec{v}_2 + 9 \hat{n} \cdot \vec{v}_2 \hat{n} \cdot \vec{v}_1 \hat{n} \times \vec{S}_1 \cdot \vec{v}_1 + \frac{73}{35} \vec{v}_1 \cdot \vec{v}_1 \hat{n} \times \vec{S}_1 \cdot \vec{v}_1 - \right. \right. \\ \left. \frac{9}{5} \vec{v}_1 \cdot \vec{v}_2 \hat{n} \times \vec{S}_1 \cdot \vec{v}_1 \right) + \frac{219}{7} \log \left( \frac{r}{R_0} \right) (\hat{n} \cdot \vec{v}_1)^2 \hat{n} \times \vec{S}_1 \cdot \vec{v}_1 + \frac{27}{5} \log \left( \frac{r}{R_0} \right) \hat{n} \cdot \vec{v}_1 \vec{S}_1 \times \vec{v}_1 \cdot \vec{v}_2 - 27 \log \left( \frac{r}{R_0} \right) \hat{n} \cdot \vec{v}_2 \\ \hat{n} \cdot \vec{v}_1 \hat{n} \times \vec{S}_1 \cdot \vec{v}_1 - \frac{219}{35} \log \left( \frac{r}{R_0} \right) \vec{v}_1 \cdot \vec{v}_1 \hat{n} \times \vec{S}_1 \cdot \vec{v}_1 + \frac{27}{5} \log \left( \frac{r}{R_0} \right) \vec{v}_1 \cdot \vec{v}_2 \hat{n} \times \vec{S}_1 \cdot \vec{v}_1 - \frac{1370}{49} (\hat{n} \cdot \vec{v}_1)^2 \hat{n} \times \vec{S}_1 \cdot \vec{v}_1 - \\ \left. \frac{319}{75} \hat{n} \cdot \vec{v}_1 \vec{S}_1 \times \vec{v}_1 \cdot \vec{v}_2 + \frac{80}{3} \hat{n} \cdot \vec{v}_2 \hat{n} \cdot \vec{v}_1 \hat{n} \times \vec{S}_1 \cdot \vec{v}_1 + \frac{6437 \vec{v}_1 \cdot \vec{v}_1 \hat{n} \times \vec{S}_1 \cdot \vec{v}_1}{1225} - \frac{319}{75} \vec{v}_1 \cdot \vec{v}_2 \hat{n} \times \vec{S}_1 \cdot \vec{v}_1 \right) \Big\}$$

$$\left\{ \text{DiagSet}[3, 1, 91], \frac{1}{r^4} \right.$$
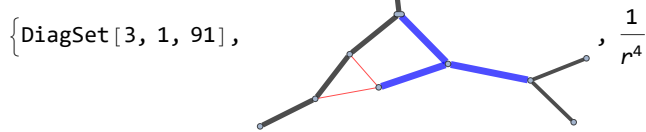

$$G^3 m_1^2 m_2 \left( \frac{1}{\epsilon_d} \left( -\frac{2}{7} (\hat{n} \cdot \vec{v}_2)^2 \hat{n} \times \vec{S}_1 \cdot \vec{v}_1 - \frac{2}{35} \hat{n} \cdot \vec{v}_2 \vec{S}_1 \times \vec{v}_1 \cdot \vec{v}_2 - \frac{6}{7} \hat{n} \cdot \vec{v}_1 \hat{n} \cdot \vec{v}_2 \hat{n} \times \vec{S}_1 \cdot \vec{v}_2 + \right. \right. \\ \left. \frac{6}{35} \vec{v}_1 \cdot \vec{v}_2 \hat{n} \times \vec{S}_1 \cdot \vec{v}_2 + \frac{2}{35} \vec{v}_2 \cdot \vec{v}_2 \hat{n} \times \vec{S}_1 \cdot \vec{v}_1 \right) + \frac{6}{7} \log\left(\frac{r}{R_0}\right) (\hat{n} \cdot \vec{v}_2)^2 \hat{n} \times \vec{S}_1 \cdot \vec{v}_1 + \\ \frac{6}{35} \log\left(\frac{r}{R_0}\right) \hat{n} \cdot \vec{v}_2 \vec{S}_1 \times \vec{v}_1 \cdot \vec{v}_2 + \frac{18}{7} \log\left(\frac{r}{R_0}\right) \hat{n} \cdot \vec{v}_1 \hat{n} \cdot \vec{v}_2 \hat{n} \times \vec{S}_1 \cdot \vec{v}_2 - \frac{18}{35} \log\left(\frac{r}{R_0}\right) \vec{v}_1 \cdot \vec{v}_2 \hat{n} \times \vec{S}_1 \cdot \vec{v}_2 - \\ \frac{6}{35} \log\left(\frac{r}{R_0}\right) \vec{v}_2 \cdot \vec{v}_2 \hat{n} \times \vec{S}_1 \cdot \vec{v}_1 - \frac{253}{49} (\hat{n} \cdot \vec{v}_2)^2 \hat{n} \times \vec{S}_1 \cdot \vec{v}_1 + \frac{1122 \hat{n} \cdot \vec{v}_2 \vec{S}_1 \times \vec{v}_1 \cdot \vec{v}_2}{1225} - \\ \left. \frac{108}{49} \hat{n} \cdot \vec{v}_1 \hat{n} \cdot \vec{v}_2 \hat{n} \times \vec{S}_1 \cdot \vec{v}_2 + \frac{204 \vec{v}_1 \cdot \vec{v}_2 \hat{n} \times \vec{S}_1 \cdot \vec{v}_2}{1225} + \frac{1643 \vec{v}_2 \cdot \vec{v}_2 \hat{n} \times \vec{S}_1 \cdot \vec{v}_1}{1225} \right\}$$

$$\left\{ \text{DiagSet}[3, 1, 92], \frac{1}{r^4} \right.$$
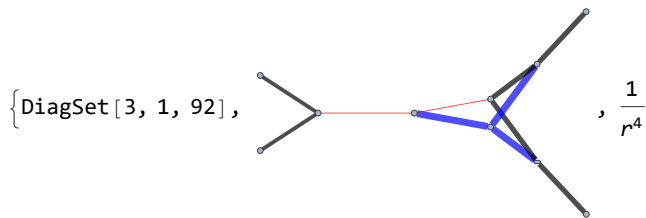

$$G^3 m_1^2 m_2 \left( \frac{\frac{83}{35} \vec{v}_1 \cdot \vec{v}_1 \hat{n} \times \vec{S}_1 \cdot \vec{v}_1 - \frac{83}{7} (\hat{n} \cdot \vec{v}_1)^2 \hat{n} \times \vec{S}_1 \cdot \vec{v}_1}{\epsilon_d} + \frac{249}{7} \log\left(\frac{r}{R_0}\right) (\hat{n} \cdot \vec{v}_1)^2 \hat{n} \times \vec{S}_1 \cdot \vec{v}_1 - \right. \\ \left. \frac{249}{35} \log\left(\frac{r}{R_0}\right) \vec{v}_1 \cdot \vec{v}_1 \hat{n} \times \vec{S}_1 \cdot \vec{v}_1 - \frac{1298}{49} (\hat{n} \cdot \vec{v}_1)^2 \hat{n} \times \vec{S}_1 \cdot \vec{v}_1 + \frac{5517 \vec{v}_1 \cdot \vec{v}_1 \hat{n} \times \vec{S}_1 \cdot \vec{v}_1}{1225} \right\}$$

$$\left\{ \text{DiagSet}[3, 1, 93], \frac{1}{r^4} \right.$$
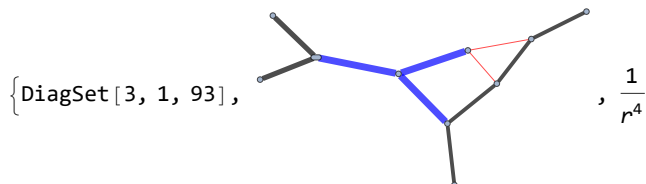

$$G^3 m_2^3 \left( \frac{1}{\epsilon_d} \left( -\frac{4}{7} (\hat{n} \cdot \vec{v}_2)^2 \hat{n} \times \vec{S}_1 \cdot \vec{v}_1 - \frac{2}{5} \hat{n} \cdot \vec{v}_2 \vec{S}_1 \times \vec{v}_1 \cdot \vec{v}_2 - \frac{22}{7} \hat{n} \cdot \vec{v}_1 \hat{n} \cdot \vec{v}_2 \hat{n} \times \vec{S}_1 \cdot \vec{v}_2 + \right. \right. \\ \left. \frac{22}{35} \vec{v}_1 \cdot \vec{v}_2 \hat{n} \times \vec{S}_1 \cdot \vec{v}_2 + \frac{4}{35} \vec{v}_2 \cdot \vec{v}_2 \hat{n} \times \vec{S}_1 \cdot \vec{v}_1 \right) + \frac{12}{7} \log\left(\frac{r}{R_0}\right) (\hat{n} \cdot \vec{v}_2)^2 \hat{n} \times \vec{S}_1 \cdot \vec{v}_1 + \\ \frac{6}{5} \log\left(\frac{r}{R_0}\right) \hat{n} \cdot \vec{v}_2 \vec{S}_1 \times \vec{v}_1 \cdot \vec{v}_2 + \frac{66}{7} \log\left(\frac{r}{R_0}\right) \hat{n} \cdot \vec{v}_1 \hat{n} \cdot \vec{v}_2 \hat{n} \times \vec{S}_1 \cdot \vec{v}_2 - \frac{66}{35} \log\left(\frac{r}{R_0}\right) \vec{v}_1 \cdot \vec{v}_2 \hat{n} \times \vec{S}_1 \cdot \vec{v}_2 - \\ \frac{12}{35} \log\left(\frac{r}{R_0}\right) \vec{v}_2 \cdot \vec{v}_2 \hat{n} \times \vec{S}_1 \cdot \vec{v}_1 - \frac{16}{49} (\hat{n} \cdot \vec{v}_2)^2 \hat{n} \times \vec{S}_1 \cdot \vec{v}_1 - \frac{14}{25} \hat{n} \cdot \vec{v}_2 \vec{S}_1 \times \vec{v}_1 \cdot \vec{v}_2 - \\ \left. \frac{228}{49} \hat{n} \cdot \vec{v}_1 \hat{n} \cdot \vec{v}_2 \hat{n} \times \vec{S}_1 \cdot \vec{v}_2 - \frac{92 \vec{v}_1 \cdot \vec{v}_2 \hat{n} \times \vec{S}_1 \cdot \vec{v}_2}{1225} + \frac{2306 \vec{v}_2 \cdot \vec{v}_2 \hat{n} \times \vec{S}_1 \cdot \vec{v}_1}{1225} \right\}$$

{DiagSet[3, 1, 94],

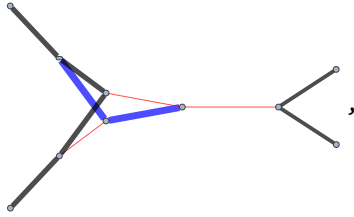

$$\begin{aligned} & \frac{1}{r^3} m_1^2 m_2 \left( -2 \log\left(\frac{r}{R_\theta}\right) \vec{S}_1 \times \vec{v}_1 \cdot \vec{v}_2 + \vec{S}_1 \times \vec{v}_1 \cdot \vec{v}_2 + \vec{S}_1 \times \vec{a}_1 \cdot \vec{v}_2 - \vec{S}_1 \times \vec{v}_1 \cdot \vec{a}_1 + \frac{192}{25} \hat{n} \times \vec{S}_1 \cdot \vec{v}_1 \hat{n} \cdot \vec{a}_1 + \frac{259}{25} \hat{n} \times \vec{S}_1 \cdot \vec{v}_1 \hat{n} \cdot \vec{v}_1 + \right. \\ & \frac{67}{25} \hat{n} \times \vec{S}_1 \cdot \vec{a}_1 \hat{n} \cdot \vec{v}_1 - 5 \hat{n} \times \vec{S}_1 \cdot \vec{v}_1 \hat{n} \cdot \vec{v}_2 - 5 \hat{n} \times \vec{S}_1 \cdot \vec{a}_1 \hat{n} \cdot \vec{v}_2 - 2 \vec{S}_1 \times \vec{a}_1 \cdot \vec{v}_2 \log\left(\frac{r}{R_\theta}\right) + 2 \vec{S}_1 \times \vec{v}_1 \cdot \vec{a}_1 \log\left(\frac{r}{R_\theta}\right) - \\ & \frac{48}{5} \hat{n} \times \vec{S}_1 \cdot \vec{v}_1 \hat{n} \cdot \vec{a}_1 \log\left(\frac{r}{R_\theta}\right) - \frac{66}{5} \hat{n} \times \vec{S}_1 \cdot \vec{v}_1 \hat{n} \cdot \vec{v}_1 \log\left(\frac{r}{R_\theta}\right) - \frac{18}{5} \hat{n} \times \vec{S}_1 \cdot \vec{a}_1 \hat{n} \cdot \vec{v}_1 \log\left(\frac{r}{R_\theta}\right) + \\ & 6 \hat{n} \times \vec{S}_1 \cdot \vec{v}_1 \hat{n} \cdot \vec{v}_2 \log\left(\frac{r}{R_\theta}\right) + 6 \hat{n} \times \vec{S}_1 \cdot \vec{a}_1 \hat{n} \cdot \vec{v}_2 \log\left(\frac{r}{R_\theta}\right) + \frac{1}{\epsilon_d} \left( \frac{2}{3} \vec{S}_1 \times \vec{v}_1 \cdot \vec{v}_2 + \frac{2}{3} \vec{S}_1 \times \vec{a}_1 \cdot \vec{v}_2 - \frac{2}{3} \vec{S}_1 \times \vec{v}_1 \cdot \vec{a}_1 + \right. \\ & \left. \frac{16}{5} \hat{n} \times \vec{S}_1 \cdot \vec{v}_1 \hat{n} \cdot \vec{a}_1 + \frac{22}{5} \hat{n} \times \vec{S}_1 \cdot \vec{v}_1 \hat{n} \cdot \vec{v}_1 + \frac{6}{5} \hat{n} \times \vec{S}_1 \cdot \vec{a}_1 \hat{n} \cdot \vec{v}_1 - 2 \hat{n} \times \vec{S}_1 \cdot \vec{v}_1 \hat{n} \cdot \vec{v}_2 - 2 \hat{n} \times \vec{S}_1 \cdot \vec{a}_1 \hat{n} \cdot \vec{v}_2 \right) \Big) G^3 + \frac{1}{r^4} \\ & m_1^2 m_2 \left( -\frac{122}{49} \hat{n} \times \vec{S}_1 \cdot \vec{v}_1 (\hat{n} \cdot \vec{v}_1)^2 + \frac{18}{7} \hat{n} \times \vec{S}_1 \cdot \vec{v}_1 \log\left(\frac{r}{R_\theta}\right) (\hat{n} \cdot \vec{v}_1)^2 + \frac{68}{25} \vec{S}_1 \times \vec{v}_1 \cdot \vec{v}_2 \hat{n} \cdot \vec{v}_1 - 16 \hat{n} \times \vec{S}_1 \cdot \vec{v}_1 \hat{n} \cdot \vec{v}_2 \hat{n} \cdot \vec{v}_1 - \right. \\ & \frac{12}{5} \vec{S}_1 \times \vec{v}_1 \cdot \vec{v}_2 \log\left(\frac{r}{R_\theta}\right) \hat{n} \cdot \vec{v}_1 + 12 \hat{n} \times \vec{S}_1 \cdot \vec{v}_1 \hat{n} \cdot \vec{v}_2 \log\left(\frac{r}{R_\theta}\right) \hat{n} \cdot \vec{v}_1 - \frac{216 \hat{n} \times \vec{S}_1 \cdot \vec{v}_1 \vec{v}_1 \cdot \vec{v}_1}{1225} + \frac{68}{25} \hat{n} \times \vec{S}_1 \cdot \vec{v}_1 \vec{v}_1 \cdot \vec{v}_2 - \\ & \frac{18}{35} \hat{n} \times \vec{S}_1 \cdot \vec{v}_1 \vec{v}_1 \cdot \vec{v}_1 \log\left(\frac{r}{R_\theta}\right) - \frac{12}{5} \hat{n} \times \vec{S}_1 \cdot \vec{v}_1 \vec{v}_1 \cdot \vec{v}_2 \log\left(\frac{r}{R_\theta}\right) + \frac{1}{\epsilon_d} \left( -\frac{6}{7} \hat{n} \times \vec{S}_1 \cdot \vec{v}_1 (\hat{n} \cdot \vec{v}_1)^2 + \right. \\ & \left. \frac{4}{5} \vec{S}_1 \times \vec{v}_1 \cdot \vec{v}_2 \hat{n} \cdot \vec{v}_1 - 4 \hat{n} \times \vec{S}_1 \cdot \vec{v}_1 \hat{n} \cdot \vec{v}_2 \hat{n} \cdot \vec{v}_1 + \frac{6}{35} \hat{n} \times \vec{S}_1 \cdot \vec{v}_1 \vec{v}_1 \cdot \vec{v}_1 + \frac{4}{5} \hat{n} \times \vec{S}_1 \cdot \vec{v}_1 \vec{v}_1 \cdot \vec{v}_2 \right) \Big) \Big) G^3 \Big\} \end{aligned}$$

{DiagSet[3, 1, 95],

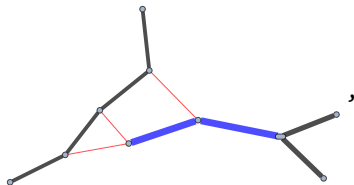

$$\begin{aligned} & \frac{1}{r^3} G^3 \left( \frac{17}{25} \hat{n} \times \vec{S}_1 \cdot \vec{v}_2 \hat{n} \cdot \vec{a}_1 - \frac{3}{5} \hat{n} \times \vec{S}_1 \cdot \vec{v}_2 \log\left(\frac{r}{R_\theta}\right) \hat{n} \cdot \vec{a}_1 + \frac{17}{25} \hat{n} \times \vec{S}_1 \cdot \vec{v}_2 \hat{n} \cdot \vec{v}_1 + \right. \\ & \frac{42}{25} \hat{n} \times \vec{S}_1 \cdot \vec{v}_1 \hat{n} \cdot \vec{v}_2 - \frac{42}{25} \hat{n} \times \vec{a}_1 \cdot \vec{S}_1 \hat{n} \cdot \vec{v}_2 + \vec{S}_1 \times \vec{v}_1 \cdot \vec{v}_2 \log\left(\frac{r}{R_\theta}\right) - \vec{a}_1 \times \vec{S}_1 \cdot \vec{v}_2 \log\left(\frac{r}{R_\theta}\right) - \\ & \frac{3}{5} \hat{n} \times \vec{S}_1 \cdot \vec{v}_2 \hat{n} \cdot \vec{v}_1 \log\left(\frac{r}{R_\theta}\right) - \frac{18}{5} \hat{n} \times \vec{S}_1 \cdot \vec{v}_1 \hat{n} \cdot \vec{v}_2 \log\left(\frac{r}{R_\theta}\right) + \frac{18}{5} \hat{n} \times \vec{a}_1 \cdot \vec{S}_1 \hat{n} \cdot \vec{v}_2 \log\left(\frac{r}{R_\theta}\right) + \frac{1}{\epsilon_d} \\ & \left( -\frac{1}{3} \vec{S}_1 \times \vec{v}_1 \cdot \vec{v}_2 + \frac{1}{3} \vec{a}_1 \times \vec{S}_1 \cdot \vec{v}_2 + \frac{1}{5} \hat{n} \times \vec{S}_1 \cdot \vec{v}_2 \hat{n} \cdot \vec{a}_1 + \frac{1}{5} \hat{n} \times \vec{S}_1 \cdot \vec{v}_2 \hat{n} \cdot \vec{v}_1 + \frac{6}{5} \hat{n} \times \vec{S}_1 \cdot \vec{v}_1 \hat{n} \cdot \vec{v}_2 - \frac{6}{5} \hat{n} \times \vec{a}_1 \cdot \vec{S}_1 \hat{n} \cdot \vec{v}_2 \right) \Big) \\ & m_2^3 + \frac{1}{r^4} G^3 \left( -4 \hat{n} \times \vec{S}_1 \cdot \vec{v}_2 (\hat{n} \cdot \vec{v}_1)^2 + 3 \hat{n} \times \vec{S}_1 \cdot \vec{v}_2 \log\left(\frac{r}{R_\theta}\right) (\hat{n} \cdot \vec{v}_1)^2 + \frac{8}{25} \vec{S}_1 \times \vec{v}_1 \cdot \vec{v}_2 \hat{n} \cdot \vec{v}_1 - 12 \hat{n} \times \vec{S}_1 \cdot \vec{v}_1 \hat{n} \cdot \vec{v}_2 \hat{n} \cdot \vec{v}_1 - \right. \\ & \frac{12}{5} \vec{S}_1 \times \vec{v}_1 \cdot \vec{v}_2 \log\left(\frac{r}{R_\theta}\right) \hat{n} \cdot \vec{v}_1 + 18 \hat{n} \times \vec{S}_1 \cdot \vec{v}_1 \hat{n} \cdot \vec{v}_2 \log\left(\frac{r}{R_\theta}\right) \hat{n} \cdot \vec{v}_1 + \frac{17}{25} \hat{n} \times \vec{S}_1 \cdot \vec{v}_2 \vec{v}_1 \cdot \vec{v}_1 + \frac{42}{25} \hat{n} \times \vec{S}_1 \cdot \vec{v}_1 \vec{v}_1 \cdot \vec{v}_2 - \\ & \frac{3}{5} \hat{n} \times \vec{S}_1 \cdot \vec{v}_2 \vec{v}_1 \cdot \vec{v}_1 \log\left(\frac{r}{R_\theta}\right) - \frac{18}{5} \hat{n} \times \vec{S}_1 \cdot \vec{v}_1 \vec{v}_1 \cdot \vec{v}_2 \log\left(\frac{r}{R_\theta}\right) + \frac{1}{\epsilon_d} \left( -(\hat{n} \times \vec{S}_1 \cdot \vec{v}_2) (\hat{n} \cdot \vec{v}_1)^2 + \right. \\ & \left. \frac{4}{5} \vec{S}_1 \times \vec{v}_1 \cdot \vec{v}_2 \hat{n} \cdot \vec{v}_1 - 6 \hat{n} \times \vec{S}_1 \cdot \vec{v}_1 \hat{n} \cdot \vec{v}_2 \hat{n} \cdot \vec{v}_1 + \frac{1}{5} \hat{n} \times \vec{S}_1 \cdot \vec{v}_2 \vec{v}_1 \cdot \vec{v}_1 + \frac{6}{5} \hat{n} \times \vec{S}_1 \cdot \vec{v}_1 \vec{v}_1 \cdot \vec{v}_2 \right) \Big) m_2^3 \Big\} \end{aligned}$$

{DiagSet[3, 1, 96],

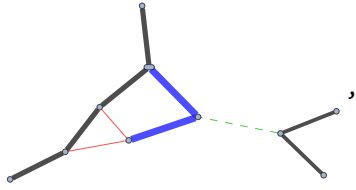

$$\begin{aligned} & \frac{1}{r^3} m_1^2 m_2 \left( -\frac{2}{5} \log\left(\frac{r}{R_\theta}\right) \frac{1}{\vec{S}_1 \times \vec{v}_1 \cdot \vec{v}_2} + \frac{83}{150} \frac{1}{\vec{S}_1 \times \vec{v}_1 \cdot \vec{v}_2} + \frac{83}{150} \frac{1}{\vec{S}_1 \times \vec{a}_1 \cdot \vec{v}_2} + \frac{71}{150} \frac{1}{\vec{S}_1 \times \vec{v}_1 \cdot \vec{a}_2} + \frac{23}{50} \hat{n} \times \vec{S}_1 \cdot \vec{v}_2 \hat{n} \cdot \vec{a}_1 + \right. \\ & \quad \frac{2}{5} \hat{n} \times \vec{S}_1 \cdot \vec{v}_1 \hat{n} \cdot \vec{a}_2 + \frac{23}{50} \hat{n} \times \vec{S}_1 \cdot \vec{v}_2 \hat{n} \cdot \vec{v}_1 + \frac{71}{50} \hat{n} \times \vec{S}_1 \cdot \vec{a}_2 \hat{n} \cdot \vec{v}_1 - \frac{2}{5} \frac{1}{\vec{S}_1 \times \vec{a}_1 \cdot \vec{v}_2} \log\left(\frac{r}{R_\theta}\right) - \frac{4}{5} \frac{1}{\vec{S}_1 \times \vec{v}_1 \cdot \vec{a}_2} \log\left(\frac{r}{R_\theta}\right) - \\ & \quad \frac{6}{5} \hat{n} \times \vec{S}_1 \cdot \vec{v}_2 \hat{n} \cdot \vec{a}_1 \log\left(\frac{r}{R_\theta}\right) - \frac{6}{5} \hat{n} \times \vec{S}_1 \cdot \vec{v}_2 \hat{n} \cdot \vec{v}_1 \log\left(\frac{r}{R_\theta}\right) - \frac{12}{5} \hat{n} \times \vec{S}_1 \cdot \vec{a}_2 \hat{n} \cdot \vec{v}_1 \log\left(\frac{r}{R_\theta}\right) + \frac{1}{\epsilon_d} \\ & \quad \left. \left( \frac{2}{15} \frac{1}{\vec{S}_1 \times \vec{v}_1 \cdot \vec{v}_2} + \frac{2}{15} \frac{1}{\vec{S}_1 \times \vec{a}_1 \cdot \vec{v}_2} + \frac{4}{15} \frac{1}{\vec{S}_1 \times \vec{v}_1 \cdot \vec{a}_2} + \frac{2}{5} \hat{n} \times \vec{S}_1 \cdot \vec{v}_2 \hat{n} \cdot \vec{a}_1 + \frac{2}{5} \hat{n} \times \vec{S}_1 \cdot \vec{v}_2 \hat{n} \cdot \vec{v}_1 + \frac{4}{5} \hat{n} \times \vec{S}_1 \cdot \vec{a}_2 \hat{n} \cdot \vec{v}_1 \right) \right) G^3 + \\ & \quad \frac{1}{r^4} m_1^2 m_2 \left( -\frac{1009}{98} \hat{n} \times \vec{S}_1 \cdot \vec{v}_2 (\hat{n} \cdot \vec{v}_1)^2 + \frac{87}{7} \hat{n} \times \vec{S}_1 \cdot \vec{v}_2 \log\left(\frac{r}{R_\theta}\right) (\hat{n} \cdot \vec{v}_1)^2 - \frac{547}{175} \vec{S}_1 \times \vec{v}_1 \cdot \vec{v}_2 \hat{n} \cdot \vec{v}_1 - \frac{106}{49} \hat{n} \times \vec{S}_1 \cdot \vec{v}_1 \right. \\ & \quad \hat{n} \cdot \vec{v}_2 \hat{n} \cdot \vec{v}_1 + \frac{19}{2} \hat{n} \times \vec{S}_1 \cdot \vec{v}_2 \hat{n} \cdot \vec{v}_2 \hat{n} \cdot \vec{v}_1 + \frac{24}{5} \vec{S}_1 \times \vec{v}_1 \cdot \vec{v}_2 \log\left(\frac{r}{R_\theta}\right) \hat{n} \cdot \vec{v}_1 + \frac{6}{7} \hat{n} \times \vec{S}_1 \cdot \vec{v}_1 \hat{n} \cdot \vec{v}_2 \log\left(\frac{r}{R_\theta}\right) \hat{n} \cdot \vec{v}_1 - \\ & \quad 12 \hat{n} \times \vec{S}_1 \cdot \vec{v}_2 \hat{n} \cdot \vec{v}_2 \log\left(\frac{r}{R_\theta}\right) \hat{n} \cdot \vec{v}_1 + 2 \hat{n} \times \vec{S}_1 \cdot \vec{v}_1 (\hat{n} \cdot \vec{v}_2)^2 + \frac{91}{50} \vec{S}_1 \times \vec{v}_1 \cdot \vec{v}_2 \hat{n} \cdot \vec{v}_2 + \frac{4247 \hat{n} \times \vec{S}_1 \cdot \vec{v}_2 \vec{v}_1 \cdot \vec{v}_1}{2450} + \\ & \quad \frac{418 \hat{n} \times \vec{S}_1 \cdot \vec{v}_1 \vec{v}_1 \cdot \vec{v}_2}{1225} - \frac{71}{50} \hat{n} \times \vec{S}_1 \cdot \vec{v}_2 \vec{v}_1 \cdot \vec{v}_2 - \frac{2}{5} \hat{n} \times \vec{S}_1 \cdot \vec{v}_1 \vec{v}_2 \cdot \vec{v}_2 - \frac{12}{5} \vec{S}_1 \times \vec{v}_1 \cdot \vec{v}_2 \hat{n} \cdot \vec{v}_2 \log\left(\frac{r}{R_\theta}\right) - \\ & \quad \frac{87}{35} \hat{n} \times \vec{S}_1 \cdot \vec{v}_2 \vec{v}_1 \cdot \vec{v}_1 \log\left(\frac{r}{R_\theta}\right) - \frac{6}{35} \hat{n} \times \vec{S}_1 \cdot \vec{v}_1 \vec{v}_1 \cdot \vec{v}_2 \log\left(\frac{r}{R_\theta}\right) + \frac{12}{5} \hat{n} \times \vec{S}_1 \cdot \vec{v}_2 \vec{v}_1 \cdot \vec{v}_2 \log\left(\frac{r}{R_\theta}\right) + \frac{1}{\epsilon_d} \\ & \quad \left. \left( -\frac{29}{7} \hat{n} \times \vec{S}_1 \cdot \vec{v}_2 (\hat{n} \cdot \vec{v}_1)^2 - \frac{8}{5} \vec{S}_1 \times \vec{v}_1 \cdot \vec{v}_2 \hat{n} \cdot \vec{v}_1 - \frac{2}{7} \hat{n} \times \vec{S}_1 \cdot \vec{v}_1 \hat{n} \cdot \vec{v}_2 \hat{n} \cdot \vec{v}_1 + 4 \hat{n} \times \vec{S}_1 \cdot \vec{v}_2 \hat{n} \cdot \vec{v}_2 \hat{n} \cdot \vec{v}_1 + \right. \right. \\ & \quad \left. \left. \frac{4}{5} \vec{S}_1 \times \vec{v}_1 \cdot \vec{v}_2 \hat{n} \cdot \vec{v}_2 + \frac{29}{35} \hat{n} \times \vec{S}_1 \cdot \vec{v}_2 \vec{v}_1 \cdot \vec{v}_1 + \frac{2}{35} \hat{n} \times \vec{S}_1 \cdot \vec{v}_1 \vec{v}_1 \cdot \vec{v}_2 - \frac{4}{5} \hat{n} \times \vec{S}_1 \cdot \vec{v}_2 \vec{v}_1 \cdot \vec{v}_2 \right) \right) G^3 \} \end{aligned}$$

{DiagSet[3, 1, 97],

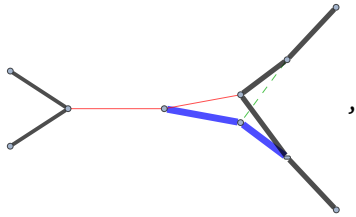

$$\begin{aligned} & \frac{1}{r^3} G^3 m_1^2 m_2 \left( \frac{-5 \hat{n} \cdot \vec{a}_1 \hat{n} \times \vec{S}_1 \cdot \vec{v}_1 + 3 \hat{n} \cdot \vec{v}_1 \hat{n} \times \vec{S}_1 \cdot \vec{a}_1 + \frac{8}{3} \vec{S}_1 \times \vec{v}_1 \cdot \vec{a}_1 - \hat{n} \cdot \vec{v}_1 \hat{n} \times \vec{S}_1 \cdot \vec{v}_1}{\epsilon_d} + \right. \\ & \quad 15 \log\left(\frac{r}{R_\theta}\right) \hat{n} \cdot \vec{a}_1 \hat{n} \times \vec{S}_1 \cdot \vec{v}_1 - 9 \log\left(\frac{r}{R_\theta}\right) \hat{n} \cdot \vec{v}_1 \hat{n} \times \vec{S}_1 \cdot \vec{a}_1 - 12 \hat{n} \cdot \vec{a}_1 \hat{n} \times \vec{S}_1 \cdot \vec{v}_1 + 20 \hat{n} \cdot \vec{v}_1 \hat{n} \times \vec{S}_1 \cdot \vec{a}_1 - \\ & \quad \left. 8 \log\left(\frac{r}{R_\theta}\right) \vec{S}_1 \times \vec{v}_1 \cdot \vec{a}_1 + 4 \vec{S}_1 \times \vec{v}_1 \cdot \vec{a}_1 + 3 \log\left(\frac{r}{R_\theta}\right) \hat{n} \cdot \vec{v}_1 \hat{n} \times \vec{S}_1 \cdot \vec{v}_1 + 6 \hat{n} \cdot \vec{v}_1 \hat{n} \times \vec{S}_1 \cdot \vec{v}_1 \right) + \frac{1}{r^4} G^3 m_1^2 m_2 \left( \frac{1}{\epsilon_d} \right. \\ & \quad \left( \frac{40}{7} (\hat{n} \cdot \vec{v}_1)^2 \hat{n} \times \vec{S}_1 \cdot \vec{v}_1 - \frac{8}{5} \hat{n} \cdot \vec{v}_1 \vec{S}_1 \times \vec{v}_1 \cdot \vec{v}_2 + 8 \hat{n} \cdot \vec{v}_2 \hat{n} \cdot \vec{v}_1 \hat{n} \times \vec{S}_1 \cdot \vec{v}_1 - \frac{8}{7} \vec{v}_1 \cdot \vec{v}_1 \hat{n} \times \vec{S}_1 \cdot \vec{v}_1 - \frac{8}{5} \vec{v}_1 \cdot \vec{v}_2 \hat{n} \times \vec{S}_1 \cdot \vec{v}_1 \right) - \\ & \quad \left. \frac{120}{7} \log\left(\frac{r}{R_\theta}\right) (\hat{n} \cdot \vec{v}_1)^2 \hat{n} \times \vec{S}_1 \cdot \vec{v}_1 + \frac{24}{5} \log\left(\frac{r}{R_\theta}\right) \hat{n} \cdot \vec{v}_1 \vec{S}_1 \times \vec{v}_1 \cdot \vec{v}_2 - 24 \log\left(\frac{r}{R_\theta}\right) \hat{n} \cdot \vec{v}_2 \hat{n} \cdot \vec{v}_1 \hat{n} \times \vec{S}_1 \cdot \vec{v}_1 + \right. \end{aligned}$$



$$\frac{24}{7} \log\left(\frac{r}{R_\theta}\right) \vec{v}_1 \cdot \vec{v}_1 \hat{n} \times \vec{S}_1 \cdot \vec{v}_1 + \frac{24}{5} \log\left(\frac{r}{R_\theta}\right) \vec{v}_1 \cdot \vec{v}_2 \hat{n} \times \vec{S}_1 \cdot \vec{v}_1 - \frac{540}{49} (\hat{n} \cdot \vec{v}_1)^2 \hat{n} \times \vec{S}_1 \cdot \vec{v}_1 - \frac{236}{25} \hat{n} \cdot \vec{v}_1 \vec{S}_1 \times \vec{v}_1 \cdot \vec{v}_2 + 52 \hat{n} \cdot \vec{v}_2 \hat{n} \cdot \vec{v}_1 \hat{n} \times \vec{S}_1 \cdot \vec{v}_1 + \frac{792}{245} \vec{v}_1 \cdot \vec{v}_1 \hat{n} \times \vec{S}_1 \cdot \vec{v}_1 - \frac{236}{25} \vec{v}_1 \cdot \vec{v}_2 \hat{n} \times \vec{S}_1 \cdot \vec{v}_1 \Big\}$$

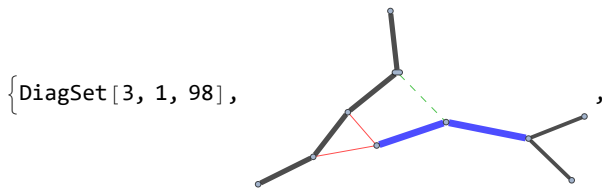

$$\frac{1}{r^3} m_1^2 m_2 \left( -\frac{3}{50} \hat{n} \times \vec{S}_1 \cdot \vec{v}_2 \hat{n} \cdot \vec{a}_2 + \frac{6}{5} \hat{n} \times \vec{S}_1 \cdot \vec{v}_2 \log\left(\frac{r}{R_\theta}\right) \hat{n} \cdot \vec{a}_2 + \frac{9}{10} \hat{n} \times \vec{S}_1 \cdot \vec{v}_2 \hat{n} \cdot \vec{v}_2 - \frac{3}{50} \hat{n} \times \vec{S}_1 \cdot \vec{a}_2 \hat{n} \cdot \vec{v}_2 + \frac{6}{5} \hat{n} \times \vec{S}_1 \cdot \vec{a}_2 \hat{n} \cdot \vec{v}_2 \log\left(\frac{r}{R_\theta}\right) + \frac{-\frac{2}{5} \hat{n} \times \vec{S}_1 \cdot \vec{v}_2 \hat{n} \cdot \vec{a}_2 - \frac{2}{5} \hat{n} \times \vec{S}_1 \cdot \vec{a}_2 \hat{n} \cdot \vec{v}_2}{\epsilon_d} \right) G^3 + \frac{1}{r^4} m_1^2 m_2 \left( \frac{253}{49} \hat{n} \times \vec{S}_1 \cdot \vec{v}_1 (\hat{n} \cdot \vec{v}_2)^2 - \frac{3}{2} \hat{n} \times \vec{S}_1 \cdot \vec{v}_2 (\hat{n} \cdot \vec{v}_2)^2 - \frac{27}{7} \hat{n} \times \vec{S}_1 \cdot \vec{v}_1 \log\left(\frac{r}{R_\theta}\right) (\hat{n} \cdot \vec{v}_2)^2 + 6 \hat{n} \times \vec{S}_1 \cdot \vec{v}_2 \log\left(\frac{r}{R_\theta}\right) (\hat{n} \cdot \vec{v}_2)^2 - \frac{639}{490} \vec{S}_1 \times \vec{v}_1 \cdot \vec{v}_2 \hat{n} \cdot \vec{v}_2 + \frac{681}{98} \hat{n} \times \vec{S}_1 \cdot \vec{v}_2 \hat{n} \cdot \vec{v}_1 \hat{n} \cdot \vec{v}_2 - \frac{3}{7} \vec{S}_1 \times \vec{v}_1 \cdot \vec{v}_2 \log\left(\frac{r}{R_\theta}\right) \hat{n} \cdot \vec{v}_2 - \frac{69}{7} \hat{n} \times \vec{S}_1 \cdot \vec{v}_2 \hat{n} \cdot \vec{v}_1 \log\left(\frac{r}{R_\theta}\right) \hat{n} \cdot \vec{v}_2 - \frac{3279 \hat{n} \times \vec{S}_1 \cdot \vec{v}_2 \vec{v}_1 \cdot \vec{v}_2}{2450} - \frac{516 \hat{n} \times \vec{S}_1 \cdot \vec{v}_1 \vec{v}_2 \cdot \vec{v}_2}{1225} + \frac{3}{50} \hat{n} \times \vec{S}_1 \cdot \vec{v}_2 \vec{v}_2 \cdot \vec{v}_2 + \frac{69}{35} \hat{n} \times \vec{S}_1 \cdot \vec{v}_2 \vec{v}_1 \cdot \vec{v}_2 \log\left(\frac{r}{R_\theta}\right) + \frac{27}{35} \hat{n} \times \vec{S}_1 \cdot \vec{v}_1 \vec{v}_2 \cdot \vec{v}_2 \log\left(\frac{r}{R_\theta}\right) - \frac{6}{5} \hat{n} \times \vec{S}_1 \cdot \vec{v}_2 \vec{v}_2 \cdot \vec{v}_2 \log\left(\frac{r}{R_\theta}\right) + \frac{1}{\epsilon_d} \left( \frac{9}{7} \hat{n} \times \vec{S}_1 \cdot \vec{v}_1 (\hat{n} \cdot \vec{v}_2)^2 - 2 \hat{n} \times \vec{S}_1 \cdot \vec{v}_2 (\hat{n} \cdot \vec{v}_2)^2 + \frac{1}{7} \vec{S}_1 \times \vec{v}_1 \cdot \vec{v}_2 \hat{n} \cdot \vec{v}_2 + \frac{23}{7} \hat{n} \times \vec{S}_1 \cdot \vec{v}_2 \hat{n} \cdot \vec{v}_1 \hat{n} \cdot \vec{v}_2 - \frac{23}{35} \hat{n} \times \vec{S}_1 \cdot \vec{v}_2 \vec{v}_1 \cdot \vec{v}_2 - \frac{9}{35} \hat{n} \times \vec{S}_1 \cdot \vec{v}_1 \vec{v}_2 \cdot \vec{v}_2 + \frac{2}{5} \hat{n} \times \vec{S}_1 \cdot \vec{v}_2 \vec{v}_2 \cdot \vec{v}_2 \right) \Big\} G^3 \Big\}$$

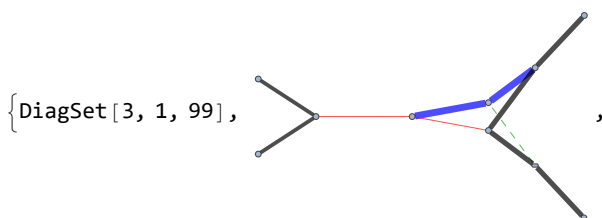

$$\frac{1}{r^3} G^3 m_1^2 m_2 \left( \frac{\frac{3}{5} \hat{n} \cdot \vec{a}_1 \hat{n} \times \vec{S}_1 \cdot \vec{v}_1 + \frac{3}{5} \hat{n} \cdot \vec{v}_1 \hat{n} \times \vec{S}_1 \cdot \vec{a}_1 - \frac{9}{5} \hat{n} \cdot \vec{v}_1 \hat{n} \times \vec{S}_1 \cdot \vec{v}_1}{\epsilon_d} - \frac{9}{5} \log\left(\frac{r}{R_\theta}\right) \hat{n} \cdot \vec{a}_1 \hat{n} \times \vec{S}_1 \cdot \vec{v}_1 - \frac{9}{5} \log\left(\frac{r}{R_\theta}\right) \hat{n} \cdot \vec{v}_1 \hat{n} \times \vec{S}_1 \cdot \vec{a}_1 - \frac{134}{25} \hat{n} \cdot \vec{a}_1 \hat{n} \times \vec{S}_1 \cdot \vec{v}_1 - \frac{134}{25} \hat{n} \cdot \vec{v}_1 \hat{n} \times \vec{S}_1 \cdot \vec{a}_1 + \frac{27}{5} \log\left(\frac{r}{R_\theta}\right) \hat{n} \cdot \vec{v}_1 \hat{n} \times \vec{S}_1 \cdot \vec{v}_1 - \frac{168}{25} \hat{n} \cdot \vec{v}_1 \hat{n} \times \vec{S}_1 \cdot \vec{v}_1 \right) + \frac{1}{r^4} G^3 m_1^2 m_2 \left( \frac{1}{\epsilon_d} \left( (\hat{n} \cdot \vec{v}_1)^2 \left( -(\hat{n} \times \vec{S}_1 \cdot \vec{v}_1) \right) - \frac{4}{5} \hat{n} \cdot \vec{v}_1 \vec{S}_1 \times \vec{v}_1 \cdot \vec{v}_2 + 4 \hat{n} \cdot \vec{v}_2 \hat{n} \cdot \vec{v}_1 \hat{n} \times \vec{S}_1 \cdot \vec{v}_1 + \frac{1}{5} \vec{v}_1 \cdot \vec{v}_1 \hat{n} \times \vec{S}_1 \cdot \vec{v}_1 - \frac{4}{5} \vec{v}_1 \cdot \vec{v}_2 \hat{n} \times \vec{S}_1 \cdot \vec{v}_1 \right) + 3 \log\left(\frac{r}{R_\theta}\right) (\hat{n} \cdot \vec{v}_1)^2 \hat{n} \times \vec{S}_1 \cdot \vec{v}_1 + \frac{12}{5} \log\left(\frac{r}{R_\theta}\right) \hat{n} \cdot \vec{v}_1 \vec{S}_1 \times \vec{v}_1 \cdot \vec{v}_2 - 12 \log\left(\frac{r}{R_\theta}\right) \hat{n} \cdot \vec{v}_2 \hat{n} \cdot \vec{v}_1 \hat{n} \times \vec{S}_1 \cdot \vec{v}_1 - \frac{3}{5} \log\left(\frac{r}{R_\theta}\right) \vec{v}_1 \cdot \vec{v}_1 \hat{n} \times \vec{S}_1 \cdot \vec{v}_1 + \frac{12}{5} \log\left(\frac{r}{R_\theta}\right) \vec{v}_1 \cdot \vec{v}_2 \hat{n} \times \vec{S}_1 \cdot \vec{v}_1 + 24 (\hat{n} \cdot \vec{v}_1)^2 \hat{n} \times \vec{S}_1 \cdot \vec{v}_1 + \right)$$

$$\frac{102}{25} \hat{n} \cdot \vec{v}_1 \vec{S}_1 \times \vec{v}_1 \cdot \vec{v}_2 - 18 \hat{n} \cdot \vec{v}_2 \hat{n} \cdot \vec{v}_1 \hat{n} \times \vec{S}_1 \cdot \vec{v}_1 - \frac{143}{25} \vec{v}_1 \cdot \vec{v}_1 \hat{n} \times \vec{S}_1 \cdot \vec{v}_1 + \frac{102}{25} \vec{v}_1 \cdot \vec{v}_2 \hat{n} \times \vec{S}_1 \cdot \vec{v}_1 \Big\}$$

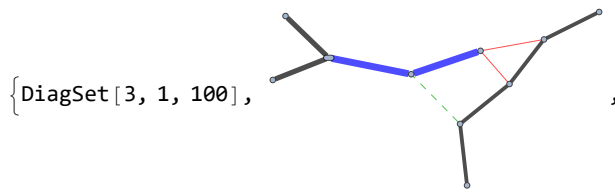

$$\begin{aligned} & \frac{1}{r^3} G^3 \left( -\log\left(\frac{r}{R_\theta}\right) \vec{S}_1 \times \vec{v}_1 \cdot \vec{v}_2 - \frac{7}{6} \vec{S}_1 \times \vec{v}_1 \cdot \vec{v}_2 + \frac{7}{6} \vec{a}_1 \times \vec{S}_1 \cdot \vec{v}_2 - \frac{7}{6} \vec{a}_2 \times \vec{S}_1 \cdot \vec{v}_1 - \frac{1}{2} \hat{n} \times \vec{S}_1 \cdot \vec{v}_2 \hat{n} \cdot \vec{a}_1 + \right. \\ & \frac{58}{25} \hat{n} \times \vec{S}_1 \cdot \vec{v}_1 \hat{n} \cdot \vec{a}_2 - \frac{1}{2} \hat{n} \times \vec{S}_1 \cdot \vec{v}_2 \hat{n} \cdot \vec{v}_1 + \frac{109}{50} \hat{n} \times \vec{a}_2 \cdot \vec{S}_1 \hat{n} \cdot \vec{v}_1 + 2 \hat{n} \times \vec{S}_1 \cdot \vec{v}_1 \hat{n} \cdot \vec{v}_2 - 2 \hat{n} \times \vec{a}_1 \cdot \vec{S}_1 \hat{n} \cdot \vec{v}_2 + \\ & \vec{a}_1 \times \vec{S}_1 \cdot \vec{v}_2 \log\left(\frac{r}{R_\theta}\right) + \vec{a}_2 \times \vec{S}_1 \cdot \vec{v}_1 \log\left(\frac{r}{R_\theta}\right) - 3 \hat{n} \times \vec{S}_1 \cdot \vec{v}_2 \hat{n} \cdot \vec{a}_1 \log\left(\frac{r}{R_\theta}\right) - \frac{12}{5} \hat{n} \times \vec{S}_1 \cdot \vec{v}_1 \hat{n} \cdot \vec{a}_2 \log\left(\frac{r}{R_\theta}\right) - \\ & 3 \hat{n} \times \vec{S}_1 \cdot \vec{v}_2 \hat{n} \cdot \vec{v}_1 \log\left(\frac{r}{R_\theta}\right) - \frac{3}{5} \hat{n} \times \vec{a}_2 \cdot \vec{S}_1 \hat{n} \cdot \vec{v}_1 \log\left(\frac{r}{R_\theta}\right) + \frac{1}{\epsilon_d} \left( \frac{1}{3} \vec{S}_1 \times \vec{v}_1 \cdot \vec{v}_2 - \frac{1}{3} \vec{a}_1 \times \vec{S}_1 \cdot \vec{v}_2 - \right. \\ & \left. \frac{1}{3} \vec{a}_2 \times \vec{S}_1 \cdot \vec{v}_1 + \hat{n} \times \vec{S}_1 \cdot \vec{v}_2 \hat{n} \cdot \vec{a}_1 + \frac{4}{5} \hat{n} \times \vec{S}_1 \cdot \vec{v}_1 \hat{n} \cdot \vec{a}_2 + \hat{n} \times \vec{S}_1 \cdot \vec{v}_2 \hat{n} \cdot \vec{v}_1 + \frac{1}{5} \hat{n} \times \vec{a}_2 \cdot \vec{S}_1 \hat{n} \cdot \vec{v}_1 \right) \Bigg) m_2^3 + \frac{1}{r^4} \\ & G^3 \left( -\frac{1}{2} \hat{n} \times \vec{S}_1 \cdot \vec{v}_2 (\hat{n} \cdot \vec{v}_1)^2 + 15 \hat{n} \times \vec{S}_1 \cdot \vec{v}_2 \log\left(\frac{r}{R_\theta}\right) (\hat{n} \cdot \vec{v}_1)^2 + 3 \vec{S}_1 \times \vec{v}_1 \cdot \vec{v}_2 \hat{n} \cdot \vec{v}_1 - 10 \hat{n} \times \vec{S}_1 \cdot \vec{v}_1 \hat{n} \cdot \vec{v}_2 \hat{n} \cdot \vec{v}_1 + \right. \\ & \frac{43}{2} \hat{n} \times \vec{S}_1 \cdot \vec{v}_2 \hat{n} \cdot \vec{v}_2 \hat{n} \cdot \vec{v}_1 + 6 \vec{S}_1 \times \vec{v}_1 \cdot \vec{v}_2 \log\left(\frac{r}{R_\theta}\right) \hat{n} \cdot \vec{v}_1 - 30 \hat{n} \times \vec{S}_1 \cdot \vec{v}_2 \hat{n} \cdot \vec{v}_2 \log\left(\frac{r}{R_\theta}\right) \hat{n} \cdot \vec{v}_1 + \\ & 6 \hat{n} \times \vec{S}_1 \cdot \vec{v}_1 (\hat{n} \cdot \vec{v}_2)^2 + \frac{83}{50} \vec{S}_1 \times \vec{v}_1 \cdot \vec{v}_2 \hat{n} \cdot \vec{v}_2 - \frac{1}{2} \hat{n} \times \vec{S}_1 \cdot \vec{v}_2 \vec{v}_1 \cdot \vec{v}_1 + 2 \hat{n} \times \vec{S}_1 \cdot \vec{v}_1 \vec{v}_1 \cdot \vec{v}_2 - \frac{39}{10} \hat{n} \times \vec{S}_1 \cdot \vec{v}_2 \vec{v}_1 \cdot \vec{v}_2 + \\ & \frac{2}{25} \hat{n} \times \vec{S}_1 \cdot \vec{v}_1 \vec{v}_2 \cdot \vec{v}_2 - 12 \hat{n} \times \vec{S}_1 \cdot \vec{v}_1 (\hat{n} \cdot \vec{v}_2)^2 \log\left(\frac{r}{R_\theta}\right) - \frac{6}{5} \vec{S}_1 \times \vec{v}_1 \cdot \vec{v}_2 \hat{n} \cdot \vec{v}_2 \log\left(\frac{r}{R_\theta}\right) - \\ & 3 \hat{n} \times \vec{S}_1 \cdot \vec{v}_2 \vec{v}_1 \cdot \vec{v}_1 \log\left(\frac{r}{R_\theta}\right) + 6 \hat{n} \times \vec{S}_1 \cdot \vec{v}_2 \vec{v}_1 \cdot \vec{v}_2 \log\left(\frac{r}{R_\theta}\right) + \frac{12}{5} \hat{n} \times \vec{S}_1 \cdot \vec{v}_1 \vec{v}_2 \cdot \vec{v}_2 \log\left(\frac{r}{R_\theta}\right) + \frac{1}{\epsilon_d} \\ & \left( -5 \hat{n} \times \vec{S}_1 \cdot \vec{v}_2 (\hat{n} \cdot \vec{v}_1)^2 - 2 \vec{S}_1 \times \vec{v}_1 \cdot \vec{v}_2 \hat{n} \cdot \vec{v}_1 + 10 \hat{n} \times \vec{S}_1 \cdot \vec{v}_2 \hat{n} \cdot \vec{v}_2 \hat{n} \cdot \vec{v}_1 + 4 \hat{n} \times \vec{S}_1 \cdot \vec{v}_1 (\hat{n} \cdot \vec{v}_2)^2 + \right. \\ & \left. \frac{2}{5} \vec{S}_1 \times \vec{v}_1 \cdot \vec{v}_2 \hat{n} \cdot \vec{v}_2 + \hat{n} \times \vec{S}_1 \cdot \vec{v}_2 \vec{v}_1 \cdot \vec{v}_1 - 2 \hat{n} \times \vec{S}_1 \cdot \vec{v}_2 \vec{v}_1 \cdot \vec{v}_2 - \frac{4}{5} \hat{n} \times \vec{S}_1 \cdot \vec{v}_1 \vec{v}_2 \cdot \vec{v}_2 \right) \Bigg) m_2^3 \Big\} \end{aligned}$$

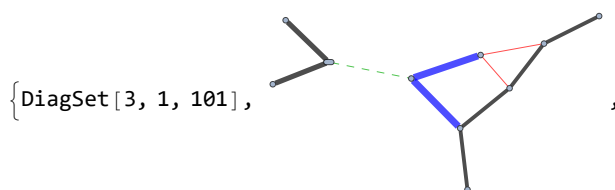

$$\begin{aligned} & \frac{1}{r^3} G^3 m_2^3 \left( \frac{\frac{1}{5} \hat{n} \cdot \vec{a}_2 \hat{n} \times \vec{S}_1 \cdot \vec{v}_2 - \frac{1}{5} \hat{n} \cdot \vec{v}_2 \hat{n} \times \vec{a}_2 \cdot \vec{S}_1 - \hat{n} \cdot \vec{v}_2 \hat{n} \times \vec{S}_1 \cdot \vec{v}_2}{\epsilon_d} - \right. \\ & \frac{3}{5} \log\left(\frac{r}{R_\theta}\right) \hat{n} \cdot \vec{a}_2 \hat{n} \times \vec{S}_1 \cdot \vec{v}_2 + \frac{3}{5} \log\left(\frac{r}{R_\theta}\right) \hat{n} \cdot \vec{v}_2 \hat{n} \times \vec{a}_2 \cdot \vec{S}_1 + \frac{109}{50} \hat{n} \cdot \vec{a}_2 \hat{n} \times \vec{S}_1 \cdot \vec{v}_2 - \\ & \left. \frac{109}{50} \hat{n} \cdot \vec{v}_2 \hat{n} \times \vec{a}_2 \cdot \vec{S}_1 + 3 \log\left(\frac{r}{R_\theta}\right) \hat{n} \cdot \vec{v}_2 \hat{n} \times \vec{S}_1 \cdot \vec{v}_2 + \frac{1}{2} \hat{n} \cdot \vec{v}_2 \hat{n} \times \vec{S}_1 \cdot \vec{v}_2 \right) + \frac{1}{r^4} G^3 m_2^3 \\ & \left( \frac{1}{\epsilon_d} \left( -\frac{51}{7} (\hat{n} \cdot \vec{v}_2)^2 \hat{n} \times \vec{S}_1 \cdot \vec{v}_2 + \hat{n} \cdot \vec{v}_2 \vec{S}_1 \times \vec{v}_1 \cdot \vec{v}_2 + 5 \hat{n} \cdot \vec{v}_1 \hat{n} \cdot \vec{v}_2 \hat{n} \times \vec{S}_1 \cdot \vec{v}_2 - \vec{v}_1 \cdot \vec{v}_2 \hat{n} \times \vec{S}_1 \cdot \vec{v}_2 + \frac{51}{35} \vec{v}_2 \cdot \vec{v}_2 \hat{n} \times \vec{S}_1 \cdot \vec{v}_2 \right) + \right. \end{aligned}$$

$$\frac{153}{7} \log\left(\frac{r}{R_0}\right) (\hat{n} \cdot \vec{v}_2)^2 \hat{n} \times \vec{S}_1 \cdot \vec{v}_2 - 3 \log\left(\frac{r}{R_0}\right) \hat{n} \cdot \vec{v}_2 \vec{S}_1 \times \vec{v}_1 \cdot \vec{v}_2 - 15 \log\left(\frac{r}{R_0}\right) \hat{n} \cdot \vec{v}_1 \hat{n} \cdot \vec{v}_2 \hat{n} \times \vec{S}_1 \cdot \vec{v}_2 +$$

$$3 \log\left(\frac{r}{R_0}\right) \vec{v}_1 \cdot \vec{v}_2 \hat{n} \times \vec{S}_1 \cdot \vec{v}_2 - \frac{153}{35} \log\left(\frac{r}{R_0}\right) \vec{v}_2 \cdot \vec{v}_2 \hat{n} \times \vec{S}_1 \cdot \vec{v}_2 - \frac{1031}{98} (\hat{n} \cdot \vec{v}_2)^2 \hat{n} \times \vec{S}_1 \cdot \vec{v}_2 -$$

$$\frac{1}{2} \hat{n} \cdot \vec{v}_2 \vec{S}_1 \times \vec{v}_1 \cdot \vec{v}_2 + \frac{1}{2} \hat{n} \cdot \vec{v}_1 \hat{n} \cdot \vec{v}_2 \hat{n} \times \vec{S}_1 \cdot \vec{v}_2 + \frac{1}{2} \vec{v}_1 \cdot \vec{v}_2 \hat{n} \times \vec{S}_1 \cdot \vec{v}_2 + \frac{1893 \vec{v}_2 \cdot \vec{v}_2 \hat{n} \times \vec{S}_1 \cdot \vec{v}_2}{2450} \Bigg\}$$

{DiagSet[3, 1, 102],

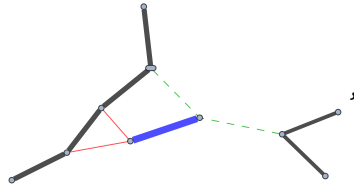

$$\frac{\hat{n} \times \vec{S}_1 \cdot \vec{a}_2 m_1^2 m_2 G^3}{6 r^2} + \frac{1}{r^3} m_1^2 m_2 \left( \frac{4}{5} \log\left(\frac{r}{R_0}\right) \vec{S}_1 \times \vec{v}_1 \cdot \vec{v}_2 - \frac{16}{25} \vec{S}_1 \times \vec{v}_1 \cdot \vec{v}_2 - \frac{16}{25} \vec{S}_1 \times \vec{a}_1 \cdot \vec{v}_2 -$$

$$\frac{29}{150} \vec{S}_1 \times \vec{v}_1 \cdot \vec{a}_2 + \frac{17}{25} \hat{n} \times \vec{S}_1 \cdot \vec{v}_1 \hat{n} \cdot \vec{a}_2 - \frac{3}{10} \hat{n} \times \vec{S}_1 \cdot \vec{a}_2 \hat{n} \cdot \vec{v}_1 + \frac{88}{25} \hat{n} \times \vec{S}_1 \cdot \vec{v}_1 \hat{n} \cdot \vec{v}_2 +$$

$$\frac{1}{2} \hat{n} \times \vec{S}_1 \cdot \vec{v}_2 \hat{n} \cdot \vec{v}_2 + \frac{88}{25} \hat{n} \times \vec{S}_1 \cdot \vec{a}_1 \hat{n} \cdot \vec{v}_2 + \frac{4}{5} \vec{S}_1 \times \vec{a}_1 \cdot \vec{v}_2 \log\left(\frac{r}{R_0}\right) + \frac{1}{5} \vec{S}_1 \times \vec{v}_1 \cdot \vec{a}_2 \log\left(\frac{r}{R_0}\right) -$$

$$\frac{3}{5} \hat{n} \times \vec{S}_1 \cdot \vec{v}_1 \hat{n} \cdot \vec{a}_2 \log\left(\frac{r}{R_0}\right) - \frac{12}{5} \hat{n} \times \vec{S}_1 \cdot \vec{v}_1 \hat{n} \cdot \vec{v}_2 \log\left(\frac{r}{R_0}\right) - \frac{12}{5} \hat{n} \times \vec{S}_1 \cdot \vec{a}_1 \hat{n} \cdot \vec{v}_2 \log\left(\frac{r}{R_0}\right) + \frac{1}{\epsilon_d}$$

$$\left( -\frac{4}{15} \vec{S}_1 \times \vec{v}_1 \cdot \vec{v}_2 - \frac{4}{15} \vec{S}_1 \times \vec{a}_1 \cdot \vec{v}_2 - \frac{1}{15} \vec{S}_1 \times \vec{v}_1 \cdot \vec{a}_2 + \frac{1}{5} \hat{n} \times \vec{S}_1 \cdot \vec{v}_1 \hat{n} \cdot \vec{a}_2 + \frac{4}{5} \hat{n} \times \vec{S}_1 \cdot \vec{v}_1 \hat{n} \cdot \vec{v}_2 + \frac{4}{5} \hat{n} \times \vec{S}_1 \cdot \vec{a}_1 \hat{n} \cdot \vec{v}_2 \right)$$

$$G^3 + \frac{1}{r^4} m_1^2 m_2 \left( \frac{3}{49} \hat{n} \times \vec{S}_1 \cdot \vec{v}_2 (\hat{n} \cdot \vec{v}_1)^2 + \frac{3}{7} \hat{n} \times \vec{S}_1 \cdot \vec{v}_2 \log\left(\frac{r}{R_0}\right) (\hat{n} \cdot \vec{v}_1)^2 + \frac{71 \vec{S}_1 \times \vec{v}_1 \cdot \vec{v}_2 \hat{n} \cdot \vec{v}_1}{1225} -$$

$$\frac{144}{49} \hat{n} \times \vec{S}_1 \cdot \vec{v}_1 \hat{n} \cdot \vec{v}_2 \hat{n} \cdot \vec{v}_1 - \frac{3}{2} \hat{n} \times \vec{S}_1 \cdot \vec{v}_2 \hat{n} \cdot \vec{v}_2 \hat{n} \cdot \vec{v}_1 + \frac{3}{35} \vec{S}_1 \times \vec{v}_1 \cdot \vec{v}_2 \log\left(\frac{r}{R_0}\right) \hat{n} \cdot \vec{v}_1 +$$

$$\frac{3}{7} \hat{n} \times \vec{S}_1 \cdot \vec{v}_1 \hat{n} \cdot \vec{v}_2 \log\left(\frac{r}{R_0}\right) \hat{n} \cdot \vec{v}_1 + 4 \hat{n} \times \vec{S}_1 \cdot \vec{v}_1 (\hat{n} \cdot \vec{v}_2)^2 - \frac{73}{50} \vec{S}_1 \times \vec{v}_1 \cdot \vec{v}_2 \hat{n} \cdot \vec{v}_2 -$$

$$\frac{1786 \hat{n} \times \vec{S}_1 \cdot \vec{v}_2 \vec{v}_1 \cdot \vec{v}_1}{1225} - \frac{71 \hat{n} \times \vec{S}_1 \cdot \vec{v}_1 \vec{v}_1 \cdot \vec{v}_2}{1225} + \frac{3}{10} \hat{n} \times \vec{S}_1 \cdot \vec{v}_2 \vec{v}_1 \cdot \vec{v}_2 - \frac{17}{25} \hat{n} \times \vec{S}_1 \cdot \vec{v}_1 \vec{v}_2 \cdot \vec{v}_2 -$$

$$\frac{1}{5} \hat{n} \times \vec{S}_1 \cdot \vec{v}_2 \vec{v}_2 \cdot \vec{v}_2 - 3 \hat{n} \times \vec{S}_1 \cdot \vec{v}_1 (\hat{n} \cdot \vec{v}_2)^2 \log\left(\frac{r}{R_0}\right) + \frac{6}{5} \vec{S}_1 \times \vec{v}_1 \cdot \vec{v}_2 \hat{n} \cdot \vec{v}_2 \log\left(\frac{r}{R_0}\right) -$$

$$\frac{3}{35} \hat{n} \times \vec{S}_1 \cdot \vec{v}_2 \vec{v}_1 \cdot \vec{v}_1 \log\left(\frac{r}{R_0}\right) - \frac{3}{35} \hat{n} \times \vec{S}_1 \cdot \vec{v}_1 \vec{v}_1 \cdot \vec{v}_2 \log\left(\frac{r}{R_0}\right) + \frac{3}{5} \hat{n} \times \vec{S}_1 \cdot \vec{v}_1 \vec{v}_2 \cdot \vec{v}_2 \log\left(\frac{r}{R_0}\right) + \frac{1}{\epsilon_d}$$

$$\left( -\frac{1}{7} \hat{n} \times \vec{S}_1 \cdot \vec{v}_2 (\hat{n} \cdot \vec{v}_1)^2 - \frac{1}{35} \vec{S}_1 \times \vec{v}_1 \cdot \vec{v}_2 \hat{n} \cdot \vec{v}_1 - \frac{1}{7} \hat{n} \times \vec{S}_1 \cdot \vec{v}_1 \hat{n} \cdot \vec{v}_2 \hat{n} \cdot \vec{v}_1 + \hat{n} \times \vec{S}_1 \cdot \vec{v}_1 (\hat{n} \cdot \vec{v}_2)^2 -$$

$$\frac{2}{5} \vec{S}_1 \times \vec{v}_1 \cdot \vec{v}_2 \hat{n} \cdot \vec{v}_2 + \frac{1}{35} \hat{n} \times \vec{S}_1 \cdot \vec{v}_2 \vec{v}_1 \cdot \vec{v}_1 + \frac{1}{35} \hat{n} \times \vec{S}_1 \cdot \vec{v}_1 \vec{v}_1 \cdot \vec{v}_2 - \frac{1}{5} \hat{n} \times \vec{S}_1 \cdot \vec{v}_1 \vec{v}_2 \cdot \vec{v}_2 \right) G^3 \Bigg\}$$

{DiagSet[3, 1, 103],

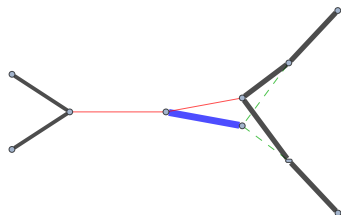

$$, \frac{m_1^2 m_2 \left( 4 \log\left(\frac{r}{R_0}\right) \hat{n} \times \vec{S}_1 \cdot \vec{a}_1 - \frac{4 \hat{n} \times \vec{S}_1 \cdot \vec{a}_1}{3 \epsilon_d} - \frac{10}{3} \hat{n} \times \vec{S}_1 \cdot \vec{a}_1 \right) G^3}{r^2} + \frac{1}{r^3}$$

$$m_1^2 m_2 \left( \frac{24}{5} \log\left(\frac{r}{R_0}\right) \vec{S}_1 \times \vec{v}_1 \cdot \vec{a}_1 - \frac{98}{75} \vec{S}_1 \times \vec{v}_1 \cdot \vec{a}_1 - \frac{109}{25} \hat{n} \times \vec{S}_1 \cdot \vec{v}_1 \hat{n} \cdot \vec{a}_1 - \frac{322}{25} \hat{n} \times \vec{S}_1 \cdot \vec{v}_1 \hat{n} \cdot \vec{v}_1 - \frac{147}{25} \hat{n} \times \vec{S}_1 \cdot \vec{a}_1 \hat{n} \cdot \vec{v}_1 + \right. \\ \left. \frac{21}{5} \hat{n} \times \vec{S}_1 \cdot \vec{v}_1 \hat{n} \cdot \vec{a}_1 \log\left(\frac{r}{R_0}\right) + \frac{138}{5} \hat{n} \times \vec{S}_1 \cdot \vec{v}_1 \hat{n} \cdot \vec{v}_1 \log\left(\frac{r}{R_0}\right) + \frac{93}{5} \hat{n} \times \vec{S}_1 \cdot \vec{a}_1 \hat{n} \cdot \vec{v}_1 \log\left(\frac{r}{R_0}\right) + \right. \\ \left. \frac{-\frac{8}{5} \vec{S}_1 \times \vec{v}_1 \cdot \vec{a}_1 - \frac{7}{5} \hat{n} \times \vec{S}_1 \cdot \vec{v}_1 \hat{n} \cdot \vec{a}_1 - \frac{46}{5} \hat{n} \times \vec{S}_1 \cdot \vec{v}_1 \hat{n} \cdot \vec{v}_1 - \frac{31}{5} \hat{n} \times \vec{S}_1 \cdot \vec{a}_1 \hat{n} \cdot \vec{v}_1}{\epsilon_d} \right) G^3 + \frac{1}{r^4}$$

$$m_1^2 m_2 \left( \frac{1002}{49} \hat{n} \times \vec{S}_1 \cdot \vec{v}_1 (\hat{n} \cdot \vec{v}_1)^2 - \frac{174}{7} \hat{n} \times \vec{S}_1 \cdot \vec{v}_1 \log\left(\frac{r}{R_0}\right) (\hat{n} \cdot \vec{v}_1)^2 + \frac{2}{25} \vec{S}_1 \times \vec{v}_1 \cdot \vec{v}_2 \hat{n} \cdot \vec{v}_1 - \hat{n} \times \vec{S}_1 \cdot \vec{v}_1 \hat{n} \cdot \vec{v}_2 \hat{n} \cdot \vec{v}_1 - \right. \\ \left. \frac{3}{5} \vec{S}_1 \times \vec{v}_1 \cdot \vec{v}_2 \log\left(\frac{r}{R_0}\right) \hat{n} \cdot \vec{v}_1 + 3 \hat{n} \times \vec{S}_1 \cdot \vec{v}_1 \hat{n} \cdot \vec{v}_2 \log\left(\frac{r}{R_0}\right) \hat{n} \cdot \vec{v}_1 - \frac{8622 \hat{n} \times \vec{S}_1 \cdot \vec{v}_1 \vec{v}_1 \cdot \vec{v}_1}{1225} + \frac{2}{25} \hat{n} \times \vec{S}_1 \cdot \vec{v}_1 \vec{v}_1 \cdot \vec{v}_2 - \right. \\ \left. 3 \hat{n} \times \vec{S}_1 \cdot \vec{v}_1 \vec{v}_2 \cdot \vec{v}_2 + \frac{174}{35} \hat{n} \times \vec{S}_1 \cdot \vec{v}_1 \vec{v}_1 \cdot \vec{v}_1 \log\left(\frac{r}{R_0}\right) - \frac{3}{5} \hat{n} \times \vec{S}_1 \cdot \vec{v}_1 \vec{v}_1 \cdot \vec{v}_2 \log\left(\frac{r}{R_0}\right) + \frac{1}{\epsilon_d} \left( \frac{58}{7} \hat{n} \times \vec{S}_1 \cdot \vec{v}_1 (\hat{n} \cdot \vec{v}_1)^2 + \right. \right. \\ \left. \left. \frac{1}{5} \vec{S}_1 \times \vec{v}_1 \cdot \vec{v}_2 \hat{n} \cdot \vec{v}_1 - \hat{n} \times \vec{S}_1 \cdot \vec{v}_1 \hat{n} \cdot \vec{v}_2 \hat{n} \cdot \vec{v}_1 - \frac{58}{35} \hat{n} \times \vec{S}_1 \cdot \vec{v}_1 \vec{v}_1 \cdot \vec{v}_1 + \frac{1}{5} \hat{n} \times \vec{S}_1 \cdot \vec{v}_1 \vec{v}_1 \cdot \vec{v}_2 \right) \right) G^3 \Big\}$$

$$\left\{ \text{DiagSet}[3, 1, 104], \right. \\ \left. \frac{1}{r^4} \right\}$$
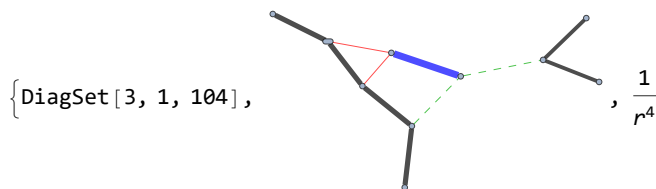

$$G^3 m_1^2 m_2 \left( \frac{\frac{48}{35} \hat{n} \cdot \vec{v}_1 \vec{S}_1 \times \vec{v}_1 \cdot \vec{v}_2 - \frac{48}{7} \hat{n} \cdot \vec{v}_2 \hat{n} \cdot \vec{v}_1 \hat{n} \times \vec{S}_1 \cdot \vec{v}_1 + \frac{48}{35} \vec{v}_1 \cdot \vec{v}_2 \hat{n} \times \vec{S}_1 \cdot \vec{v}_1}{\epsilon_d} - \right. \\ \left. \frac{144}{35} \log\left(\frac{r}{R_0}\right) \hat{n} \cdot \vec{v}_1 \vec{S}_1 \times \vec{v}_1 \cdot \vec{v}_2 + \frac{144}{7} \log\left(\frac{r}{R_0}\right) \hat{n} \cdot \vec{v}_2 \hat{n} \cdot \vec{v}_1 \hat{n} \times \vec{S}_1 \cdot \vec{v}_1 - \frac{144}{35} \log\left(\frac{r}{R_0}\right) \vec{v}_1 \cdot \vec{v}_2 \hat{n} \times \vec{S}_1 \cdot \vec{v}_1 + \right. \\ \left. \frac{6392 \hat{n} \cdot \vec{v}_1 \vec{S}_1 \times \vec{v}_1 \cdot \vec{v}_2}{1225} - \frac{1424}{49} \hat{n} \cdot \vec{v}_2 \hat{n} \cdot \vec{v}_1 \hat{n} \times \vec{S}_1 \cdot \vec{v}_1 + \frac{6392 \vec{v}_1 \cdot \vec{v}_2 \hat{n} \times \vec{S}_1 \cdot \vec{v}_1}{1225} \right) \Big\}$$

$$\left\{ \text{DiagSet}[3, 1, 105], \right. \\ \left. \frac{1}{r^4} \right\}$$
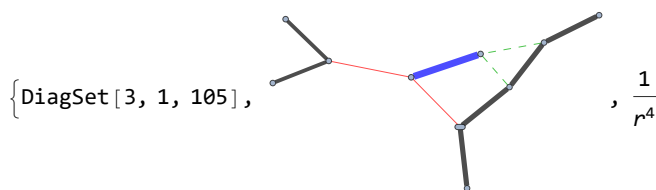

$$G^3 m_1^2 m_2 \left( \frac{24 (\hat{n} \cdot \vec{v}_1)^2 \hat{n} \times \vec{S}_1 \cdot \vec{v}_1 - \frac{24}{5} \vec{v}_1 \cdot \vec{v}_1 \hat{n} \times \vec{S}_1 \cdot \vec{v}_1}{\epsilon_d} - 72 \log\left(\frac{r}{R_0}\right) (\hat{n} \cdot \vec{v}_1)^2 \hat{n} \times \vec{S}_1 \cdot \vec{v}_1 + \right. \\ \left. \frac{72}{5} \log\left(\frac{r}{R_0}\right) \vec{v}_1 \cdot \vec{v}_1 \hat{n} \times \vec{S}_1 \cdot \vec{v}_1 + 32 (\hat{n} \cdot \vec{v}_1)^2 \hat{n} \times \vec{S}_1 \cdot \vec{v}_1 - \frac{208}{25} \vec{v}_1 \cdot \vec{v}_1 \hat{n} \times \vec{S}_1 \cdot \vec{v}_1 \right) \Big\}$$

$$\left\{ \text{DiagSet}[3, 1, 106], \right. \\ \left. \right\}$$
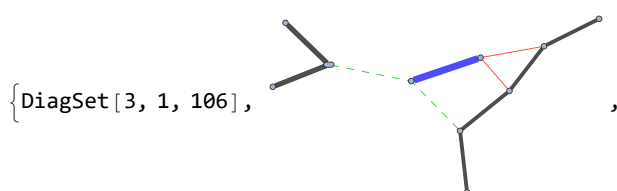

$$\begin{aligned}
 & \frac{G^3 \left( -\log\left(\frac{r}{R_\theta}\right) \hat{n} \times \vec{a}_2 \cdot \vec{S}_1 + \frac{\hat{n} \times \vec{a}_2 \cdot \vec{S}_1}{3 \in_d} + \frac{1}{6} \hat{n} \times \vec{a}_2 \cdot \vec{S}_1 \right) m_2^3}{r^2} + \frac{1}{r^3} G^3 \left( \frac{4}{5} \log\left(\frac{r}{R_\theta}\right) \vec{S}_1 \times \vec{v}_1 \cdot \vec{v}_2 - \frac{16}{25} \vec{S}_1 \times \vec{v}_1 \cdot \vec{v}_2 + \frac{16}{25} \vec{a}_1 \times \vec{S}_1 \cdot \vec{v}_2 + \right. \\
 & \frac{1}{6} \vec{a}_2 \times \vec{S}_1 \cdot \vec{v}_1 - \frac{3}{2} \hat{n} \times \vec{a}_2 \cdot \vec{S}_1 \hat{n} \cdot \vec{v}_1 + \frac{88}{25} \hat{n} \times \vec{S}_1 \cdot \vec{v}_1 \hat{n} \cdot \vec{v}_2 - \frac{43}{50} \hat{n} \times \vec{S}_1 \cdot \vec{v}_2 \hat{n} \cdot \vec{v}_2 - \frac{88}{25} \hat{n} \times \vec{a}_1 \cdot \vec{S}_1 \hat{n} \cdot \vec{v}_2 - \\
 & \frac{4}{5} \vec{a}_1 \times \vec{S}_1 \cdot \vec{v}_2 \log\left(\frac{r}{R_\theta}\right) - \vec{a}_2 \times \vec{S}_1 \cdot \vec{v}_1 \log\left(\frac{r}{R_\theta}\right) + 3 \hat{n} \times \vec{a}_2 \cdot \vec{S}_1 \hat{n} \cdot \vec{v}_1 \log\left(\frac{r}{R_\theta}\right) - \frac{12}{5} \hat{n} \times \vec{S}_1 \cdot \vec{v}_1 \hat{n} \cdot \vec{v}_2 \log\left(\frac{r}{R_\theta}\right) + \\
 & \frac{6}{5} \hat{n} \times \vec{S}_1 \cdot \vec{v}_2 \hat{n} \cdot \vec{v}_2 \log\left(\frac{r}{R_\theta}\right) + \frac{12}{5} \hat{n} \times \vec{a}_1 \cdot \vec{S}_1 \hat{n} \cdot \vec{v}_2 \log\left(\frac{r}{R_\theta}\right) + \frac{1}{\in_d} \left( -\frac{4}{15} \vec{S}_1 \times \vec{v}_1 \cdot \vec{v}_2 + \frac{4}{15} \vec{a}_1 \times \vec{S}_1 \cdot \vec{v}_2 + \right. \\
 & \left. \frac{1}{3} \vec{a}_2 \times \vec{S}_1 \cdot \vec{v}_1 - \hat{n} \times \vec{a}_2 \cdot \vec{S}_1 \hat{n} \cdot \vec{v}_1 + \frac{4}{5} \hat{n} \times \vec{S}_1 \cdot \vec{v}_1 \hat{n} \cdot \vec{v}_2 - \frac{2}{5} \hat{n} \times \vec{S}_1 \cdot \vec{v}_2 \hat{n} \cdot \vec{v}_2 - \frac{4}{5} \hat{n} \times \vec{a}_1 \cdot \vec{S}_1 \hat{n} \cdot \vec{v}_2 \right) \Big) m_2^3 + \\
 & \frac{1}{r^4} G^3 \left( \hat{n} \times \vec{S}_1 \cdot \vec{v}_2 (\hat{n} \cdot \vec{v}_2)^2 + \frac{43}{50} \vec{S}_1 \times \vec{v}_1 \cdot \vec{v}_2 \hat{n} \cdot \vec{v}_2 - 20 \hat{n} \times \vec{S}_1 \cdot \vec{v}_1 \hat{n} \cdot \vec{v}_1 \hat{n} \cdot \vec{v}_2 + \frac{11}{2} \hat{n} \times \vec{S}_1 \cdot \vec{v}_2 \hat{n} \cdot \vec{v}_1 \hat{n} \cdot \vec{v}_2 - \right. \\
 & \frac{6}{5} \vec{S}_1 \times \vec{v}_1 \cdot \vec{v}_2 \log\left(\frac{r}{R_\theta}\right) \hat{n} \cdot \vec{v}_2 + 12 \hat{n} \times \vec{S}_1 \cdot \vec{v}_1 \hat{n} \cdot \vec{v}_1 \log\left(\frac{r}{R_\theta}\right) \hat{n} \cdot \vec{v}_2 - \\
 & 6 \hat{n} \times \vec{S}_1 \cdot \vec{v}_2 \hat{n} \cdot \vec{v}_1 \log\left(\frac{r}{R_\theta}\right) \hat{n} \cdot \vec{v}_2 + \frac{83}{25} \vec{S}_1 \times \vec{v}_1 \cdot \vec{v}_2 \hat{n} \cdot \vec{v}_1 + \frac{73}{25} \hat{n} \times \vec{S}_1 \cdot \vec{v}_1 \vec{v}_1 \cdot \vec{v}_2 - \frac{43}{50} \hat{n} \times \vec{S}_1 \cdot \vec{v}_2 \vec{v}_1 \cdot \vec{v}_2 - \\
 & \frac{12}{5} \hat{n} \times \vec{S}_1 \cdot \vec{v}_2 \vec{v}_2 \cdot \vec{v}_2 - \frac{12}{5} \vec{S}_1 \times \vec{v}_1 \cdot \vec{v}_2 \hat{n} \cdot \vec{v}_1 \log\left(\frac{r}{R_\theta}\right) - \frac{12}{5} \hat{n} \times \vec{S}_1 \cdot \vec{v}_1 \vec{v}_1 \cdot \vec{v}_2 \log\left(\frac{r}{R_\theta}\right) + \\
 & \frac{6}{5} \hat{n} \times \vec{S}_1 \cdot \vec{v}_2 \vec{v}_1 \cdot \vec{v}_2 \log\left(\frac{r}{R_\theta}\right) + \frac{1}{\in_d} \left( \frac{4}{5} \vec{S}_1 \times \vec{v}_1 \cdot \vec{v}_2 \hat{n} \cdot \vec{v}_1 - 4 \hat{n} \times \vec{S}_1 \cdot \vec{v}_1 \hat{n} \cdot \vec{v}_2 \hat{n} \cdot \vec{v}_1 + \right. \\
 & \left. 2 \hat{n} \times \vec{S}_1 \cdot \vec{v}_2 \hat{n} \cdot \vec{v}_2 \hat{n} \cdot \vec{v}_1 + \frac{2}{5} \vec{S}_1 \times \vec{v}_1 \cdot \vec{v}_2 \hat{n} \cdot \vec{v}_2 + \frac{4}{5} \hat{n} \times \vec{S}_1 \cdot \vec{v}_1 \vec{v}_1 \cdot \vec{v}_2 - \frac{2}{5} \hat{n} \times \vec{S}_1 \cdot \vec{v}_2 \vec{v}_1 \cdot \vec{v}_2 \right) \Big) m_2^3 \Big\}
 \end{aligned}$$

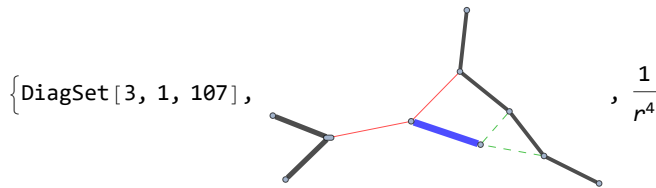

$$\begin{aligned}
 & G^3 m_2^3 \left( \frac{40 (\hat{n} \cdot \vec{v}_2)^2 \hat{n} \times \vec{S}_1 \cdot \vec{v}_1 - 16 \hat{n} \cdot \vec{v}_2 \vec{S}_1 \times \vec{v}_1 \cdot \vec{v}_2 - 8 \vec{v}_2 \cdot \vec{v}_2 \hat{n} \times \vec{S}_1 \cdot \vec{v}_1}{\in_d} - \right. \\
 & 120 \log\left(\frac{r}{R_\theta}\right) (\hat{n} \cdot \vec{v}_2)^2 \hat{n} \times \vec{S}_1 \cdot \vec{v}_1 + 48 \log\left(\frac{r}{R_\theta}\right) \hat{n} \cdot \vec{v}_2 \vec{S}_1 \times \vec{v}_1 \cdot \vec{v}_2 + 24 \log\left(\frac{r}{R_\theta}\right) \vec{v}_2 \cdot \vec{v}_2 \hat{n} \times \vec{S}_1 \cdot \vec{v}_1 + \\
 & \left. 64 (\hat{n} \cdot \vec{v}_2)^2 \hat{n} \times \vec{S}_1 \cdot \vec{v}_1 - 16 \hat{n} \cdot \vec{v}_2 \vec{S}_1 \times \vec{v}_1 \cdot \vec{v}_2 - 16 \vec{v}_2 \cdot \vec{v}_2 \hat{n} \times \vec{S}_1 \cdot \vec{v}_1 \right\}
 \end{aligned}$$

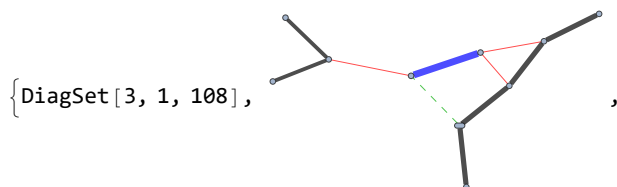

$$\begin{aligned}
 & \frac{1}{r^2} m_1^2 m_2 \left( 4 \log\left(\frac{r}{R_\theta}\right) \hat{n} \times \vec{S}_1 \cdot \vec{a}_1 - \frac{10}{3} \hat{n} \times \vec{S}_1 \cdot \vec{a}_1 - \frac{5}{3} \hat{n} \times \vec{S}_1 \cdot \vec{v}_1 - \frac{5}{3} \hat{n} \times \vec{S}_1 \cdot \vec{a}_1 + \right. \\
 & \left. 2 \hat{n} \times \vec{S}_1 \cdot \vec{v}_1 \log\left(\frac{r}{R_\theta}\right) + 2 \hat{n} \times \vec{S}_1 \cdot \vec{a}_1 \log\left(\frac{r}{R_\theta}\right) + \frac{-\frac{4}{3} \hat{n} \times \vec{S}_1 \cdot \vec{a}_1 - \frac{2}{3} \hat{n} \times \vec{S}_1 \cdot \vec{v}_1 - \frac{2}{3} \hat{n} \times \vec{S}_1 \cdot \vec{a}_1}{\in_d} \right) G^3 + \frac{1}{r^3} m_1^2 m_2
 \end{aligned}$$

$$\begin{aligned}
& \left( -2 \log \left( \frac{r}{R_\theta} \right) \frac{1}{\vec{S}_1 \cdot \vec{v}_1 \cdot \vec{v}_2} + \frac{5}{3} \frac{1}{\vec{S}_1 \cdot \vec{v}_1 \cdot \vec{v}_2} + \frac{5}{3} \frac{1}{\vec{S}_1 \cdot \vec{a}_1 \cdot \vec{v}_2} + \frac{23}{75} \frac{1}{\vec{S}_1 \cdot \vec{v}_1 \cdot \vec{a}_1} + \frac{63}{25} \frac{1}{\hat{n} \times \vec{S}_1 \cdot \vec{v}_1 \cdot \hat{n} \cdot \vec{a}_1} + \frac{109}{25} \frac{1}{\hat{n} \times \vec{S}_1 \cdot \vec{v}_1 \cdot \hat{n} \cdot \vec{v}_1} + \right. \\
& \frac{126}{25} \frac{1}{\hat{n} \times \vec{S}_1 \cdot \vec{a}_1 \cdot \hat{n} \cdot \vec{v}_1} - 7 \frac{1}{\hat{n} \times \vec{S}_1 \cdot \vec{v}_1 \cdot \hat{n} \cdot \vec{v}_2} - 7 \frac{1}{\hat{n} \times \vec{S}_1 \cdot \vec{a}_1 \cdot \hat{n} \cdot \vec{v}_2} - 2 \frac{1}{\vec{S}_1 \cdot \vec{a}_1 \cdot \vec{v}_2} \log \left( \frac{r}{R_\theta} \right) - \frac{4}{5} \frac{1}{\vec{S}_1 \cdot \vec{v}_1 \cdot \vec{a}_1} \log \left( \frac{r}{R_\theta} \right) - \\
& \frac{12}{5} \frac{1}{\hat{n} \times \vec{S}_1 \cdot \vec{v}_1 \cdot \hat{n} \cdot \vec{a}_1} \log \left( \frac{r}{R_\theta} \right) - \frac{21}{5} \frac{1}{\hat{n} \times \vec{S}_1 \cdot \vec{v}_1 \cdot \hat{n} \cdot \vec{v}_1} \log \left( \frac{r}{R_\theta} \right) - \frac{24}{5} \frac{1}{\hat{n} \times \vec{S}_1 \cdot \vec{a}_1 \cdot \hat{n} \cdot \vec{v}_1} \log \left( \frac{r}{R_\theta} \right) + \\
& 6 \frac{1}{\hat{n} \times \vec{S}_1 \cdot \vec{v}_1 \cdot \hat{n} \cdot \vec{v}_2} \log \left( \frac{r}{R_\theta} \right) + 6 \frac{1}{\hat{n} \times \vec{S}_1 \cdot \vec{a}_1 \cdot \hat{n} \cdot \vec{v}_2} \log \left( \frac{r}{R_\theta} \right) + \frac{1}{\epsilon_d} \left( \frac{2}{3} \frac{1}{\vec{S}_1 \cdot \vec{v}_1 \cdot \vec{v}_2} + \frac{2}{3} \frac{1}{\vec{S}_1 \cdot \vec{a}_1 \cdot \vec{v}_2} + \frac{4}{15} \frac{1}{\vec{S}_1 \cdot \vec{v}_1 \cdot \vec{a}_1} + \right. \\
& \left. \frac{4}{5} \frac{1}{\hat{n} \times \vec{S}_1 \cdot \vec{v}_1 \cdot \hat{n} \cdot \vec{a}_1} + \frac{7}{5} \frac{1}{\hat{n} \times \vec{S}_1 \cdot \vec{v}_1 \cdot \hat{n} \cdot \vec{v}_1} + \frac{8}{5} \frac{1}{\hat{n} \times \vec{S}_1 \cdot \vec{a}_1 \cdot \hat{n} \cdot \vec{v}_1} - 2 \frac{1}{\hat{n} \times \vec{S}_1 \cdot \vec{v}_1 \cdot \hat{n} \cdot \vec{v}_2} - 2 \frac{1}{\hat{n} \times \vec{S}_1 \cdot \vec{a}_1 \cdot \hat{n} \cdot \vec{v}_2} \right) \Big) G^3 + \\
& \frac{1}{r^4} m_1^2 m_2 \left( -\frac{404}{49} \frac{1}{\hat{n} \times \vec{S}_1 \cdot \vec{v}_1} (\hat{n} \cdot \vec{v}_1)^2 + \frac{51}{7} \frac{1}{\hat{n} \times \vec{S}_1 \cdot \vec{v}_1} \log \left( \frac{r}{R_\theta} \right) (\hat{n} \cdot \vec{v}_1)^2 - \frac{63}{25} \frac{1}{\vec{S}_1 \cdot \vec{v}_1 \cdot \vec{v}_2} \hat{n} \cdot \vec{v}_1 + \right. \\
& 15 \frac{1}{\hat{n} \times \vec{S}_1 \cdot \vec{v}_1 \cdot \hat{n} \cdot \vec{v}_2} \hat{n} \cdot \vec{v}_1 + \frac{12}{5} \frac{1}{\vec{S}_1 \cdot \vec{v}_1 \cdot \vec{v}_2} \log \left( \frac{r}{R_\theta} \right) \hat{n} \cdot \vec{v}_1 - 12 \frac{1}{\hat{n} \times \vec{S}_1 \cdot \vec{v}_1 \cdot \hat{n} \cdot \vec{v}_2} \log \left( \frac{r}{R_\theta} \right) \hat{n} \cdot \vec{v}_1 - \\
& \frac{1049}{2450} \frac{1}{\hat{n} \times \vec{S}_1 \cdot \vec{v}_1 \cdot \vec{v}_1 \cdot \vec{v}_1} - \frac{63}{25} \frac{1}{\hat{n} \times \vec{S}_1 \cdot \vec{v}_1 \cdot \vec{v}_1 \cdot \vec{v}_2} - \frac{9}{10} \frac{1}{\hat{n} \times \vec{S}_1 \cdot \vec{v}_1 \cdot \vec{v}_2 \cdot \vec{v}_2} - \frac{51}{35} \frac{1}{\hat{n} \times \vec{S}_1 \cdot \vec{v}_1 \cdot \vec{v}_1 \cdot \vec{v}_1} \log \left( \frac{r}{R_\theta} \right) + \\
& \frac{12}{5} \frac{1}{\hat{n} \times \vec{S}_1 \cdot \vec{v}_1 \cdot \vec{v}_1 \cdot \vec{v}_2} \log \left( \frac{r}{R_\theta} \right) + \frac{1}{\epsilon_d} \left( -\frac{17}{7} \frac{1}{\hat{n} \times \vec{S}_1 \cdot \vec{v}_1} (\hat{n} \cdot \vec{v}_1)^2 - \frac{4}{5} \frac{1}{\vec{S}_1 \cdot \vec{v}_1 \cdot \vec{v}_2} \hat{n} \cdot \vec{v}_1 + \right. \\
& \left. 4 \frac{1}{\hat{n} \times \vec{S}_1 \cdot \vec{v}_1 \cdot \hat{n} \cdot \vec{v}_2} \hat{n} \cdot \vec{v}_1 + \frac{17}{35} \frac{1}{\hat{n} \times \vec{S}_1 \cdot \vec{v}_1 \cdot \vec{v}_1 \cdot \vec{v}_1} - \frac{4}{5} \frac{1}{\hat{n} \times \vec{S}_1 \cdot \vec{v}_1 \cdot \vec{v}_1 \cdot \vec{v}_2} \right) \Big) G^3 \Big\}
\end{aligned}$$

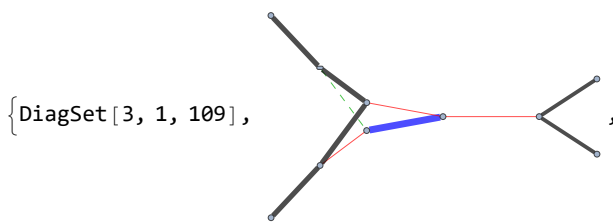

$$\begin{aligned}
& \frac{1}{r^2} m_1^2 m_2 \left( 24 \log \left( \frac{r}{R_\theta} \right) \frac{1}{\hat{n} \times \vec{S}_1 \cdot \vec{a}_1} - 20 \frac{1}{\hat{n} \times \vec{S}_1 \cdot \vec{a}_1} - 10 \frac{1}{\hat{n} \times \vec{S}_1 \cdot \vec{v}_1} - 10 \frac{1}{\hat{n} \times \vec{S}_1 \cdot \vec{a}_1} + \right. \\
& 12 \frac{1}{\hat{n} \times \vec{S}_1 \cdot \vec{v}_1} \log \left( \frac{r}{R_\theta} \right) + 12 \frac{1}{\hat{n} \times \vec{S}_1 \cdot \vec{a}_1} \log \left( \frac{r}{R_\theta} \right) + \frac{-8 \frac{1}{\hat{n} \times \vec{S}_1 \cdot \vec{a}_1} - 4 \frac{1}{\hat{n} \times \vec{S}_1 \cdot \vec{v}_1} - 4 \frac{1}{\hat{n} \times \vec{S}_1 \cdot \vec{a}_1}}{\epsilon_d} \Big) G^3 + \\
& \frac{1}{r^3} m_1^2 m_2 \left( \frac{-2 \frac{1}{\hat{n} \times \vec{S}_1 \cdot \vec{v}_1 \cdot \hat{n} \cdot \vec{a}_1} - 2 \frac{1}{\hat{n} \times \vec{S}_1 \cdot \vec{v}_1 \cdot \hat{n} \cdot \vec{v}_1} - 2 \frac{1}{\hat{n} \times \vec{S}_1 \cdot \vec{a}_1 \cdot \hat{n} \cdot \vec{v}_1}}{\epsilon_d} + 6 \frac{1}{\hat{n} \times \vec{S}_1 \cdot \vec{v}_1 \cdot \hat{n} \cdot \vec{a}_1} \log \left( \frac{r}{R_\theta} \right) + \right. \\
& \left. 6 \frac{1}{\hat{n} \times \vec{S}_1 \cdot \vec{v}_1 \cdot \hat{n} \cdot \vec{v}_1} \log \left( \frac{r}{R_\theta} \right) + 6 \frac{1}{\hat{n} \times \vec{S}_1 \cdot \vec{a}_1 \cdot \hat{n} \cdot \vec{v}_1} \log \left( \frac{r}{R_\theta} \right) \right) G^3 + \frac{1}{r^4} \\
& m_1^2 m_2 \left( 8 \frac{1}{\hat{n} \times \vec{S}_1 \cdot \vec{v}_1} (\hat{n} \cdot \vec{v}_1)^2 - 12 \frac{1}{\hat{n} \times \vec{S}_1 \cdot \vec{v}_1} \log \left( \frac{r}{R_\theta} \right) (\hat{n} \cdot \vec{v}_1)^2 - \frac{7}{25} \frac{1}{\vec{S}_1 \cdot \vec{v}_1 \cdot \vec{v}_2} \hat{n} \cdot \vec{v}_1 + 2 \frac{1}{\hat{n} \times \vec{S}_1 \cdot \vec{v}_1 \cdot \hat{n} \cdot \vec{v}_2} \hat{n} \cdot \vec{v}_1 + \right. \\
& \frac{3}{5} \frac{1}{\vec{S}_1 \cdot \vec{v}_1 \cdot \vec{v}_2} \log \left( \frac{r}{R_\theta} \right) \hat{n} \cdot \vec{v}_1 - 3 \frac{1}{\hat{n} \times \vec{S}_1 \cdot \vec{v}_1 \cdot \hat{n} \cdot \vec{v}_2} \log \left( \frac{r}{R_\theta} \right) \hat{n} \cdot \vec{v}_1 + \frac{89}{50} \frac{1}{\hat{n} \times \vec{S}_1 \cdot \vec{v}_1 \cdot \vec{v}_1 \cdot \vec{v}_1} - \\
& \frac{7}{25} \frac{1}{\hat{n} \times \vec{S}_1 \cdot \vec{v}_1 \cdot \vec{v}_1 \cdot \vec{v}_2} + \frac{3}{2} \frac{1}{\hat{n} \times \vec{S}_1 \cdot \vec{v}_1 \cdot \vec{v}_2 \cdot \vec{v}_2} + \frac{12}{5} \frac{1}{\hat{n} \times \vec{S}_1 \cdot \vec{v}_1 \cdot \vec{v}_1 \cdot \vec{v}_1} \log \left( \frac{r}{R_\theta} \right) + \frac{3}{5} \frac{1}{\hat{n} \times \vec{S}_1 \cdot \vec{v}_1 \cdot \vec{v}_1 \cdot \vec{v}_2} \log \left( \frac{r}{R_\theta} \right) + \frac{1}{\epsilon_d} \\
& \left. \left( 4 \frac{1}{\hat{n} \times \vec{S}_1 \cdot \vec{v}_1} (\hat{n} \cdot \vec{v}_1)^2 - \frac{1}{5} \frac{1}{\vec{S}_1 \cdot \vec{v}_1 \cdot \vec{v}_2} \hat{n} \cdot \vec{v}_1 + \hat{n} \times \vec{S}_1 \cdot \vec{v}_1 \cdot \hat{n} \cdot \vec{v}_2 \hat{n} \cdot \vec{v}_1 - \frac{4}{5} \frac{1}{\hat{n} \times \vec{S}_1 \cdot \vec{v}_1 \cdot \vec{v}_1 \cdot \vec{v}_1} - \frac{1}{5} \frac{1}{\hat{n} \times \vec{S}_1 \cdot \vec{v}_1 \cdot \vec{v}_1 \cdot \vec{v}_2} \right) \right) G^3 \Big\}
\end{aligned}$$

{DiagSet[3, 1, 110],

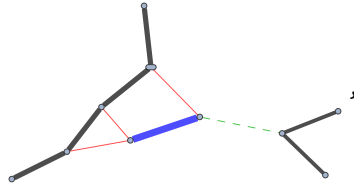

$$\begin{aligned} & \frac{1}{r^3} m_1^2 m_2 \left( -\frac{8}{5} \log\left(\frac{r}{R_\theta}\right) \vec{S}_1 \times \vec{v}_1 \cdot \vec{v}_2 + \frac{26}{75} \vec{S}_1 \times \vec{v}_1 \cdot \vec{v}_2 + \frac{26}{75} \vec{S}_1 \times \vec{a}_1 \cdot \vec{v}_2 + \frac{26}{75} \vec{S}_1 \times \vec{v}_1 \cdot \vec{a}_2 - \frac{106}{25} \hat{n} \times \vec{S}_1 \cdot \vec{v}_1 \hat{n} \cdot \vec{a}_2 - \right. \\ & \quad \frac{106}{25} \hat{n} \times \vec{S}_1 \cdot \vec{v}_1 \hat{n} \cdot \vec{v}_2 - \frac{106}{25} \hat{n} \times \vec{S}_1 \cdot \vec{a}_1 \hat{n} \cdot \vec{v}_2 - \frac{8}{5} \vec{S}_1 \times \vec{a}_1 \cdot \vec{v}_2 \log\left(\frac{r}{R_\theta}\right) - \frac{8}{5} \vec{S}_1 \times \vec{v}_1 \cdot \vec{a}_2 \log\left(\frac{r}{R_\theta}\right) + \\ & \quad \frac{24}{5} \hat{n} \times \vec{S}_1 \cdot \vec{v}_1 \hat{n} \cdot \vec{a}_2 \log\left(\frac{r}{R_\theta}\right) + \frac{24}{5} \hat{n} \times \vec{S}_1 \cdot \vec{v}_1 \hat{n} \cdot \vec{v}_2 \log\left(\frac{r}{R_\theta}\right) + \frac{24}{5} \hat{n} \times \vec{S}_1 \cdot \vec{a}_1 \hat{n} \cdot \vec{v}_2 \log\left(\frac{r}{R_\theta}\right) + \frac{1}{\epsilon_d} \\ & \quad \left. \left( \frac{8}{15} \vec{S}_1 \times \vec{v}_1 \cdot \vec{v}_2 + \frac{8}{15} \vec{S}_1 \times \vec{a}_1 \cdot \vec{v}_2 + \frac{8}{15} \vec{S}_1 \times \vec{v}_1 \cdot \vec{a}_2 - \frac{8}{5} \hat{n} \times \vec{S}_1 \cdot \vec{v}_1 \hat{n} \cdot \vec{a}_2 - \frac{8}{5} \hat{n} \times \vec{S}_1 \cdot \vec{v}_1 \hat{n} \cdot \vec{v}_2 - \frac{8}{5} \hat{n} \times \vec{S}_1 \cdot \vec{a}_1 \hat{n} \cdot \vec{v}_2 \right) \right) G^3 + \\ & \frac{1}{r^4} m_1^2 m_2 \left( -26 \hat{n} \times \vec{S}_1 \cdot \vec{v}_1 (\hat{n} \cdot \vec{v}_2)^2 + 24 \hat{n} \times \vec{S}_1 \cdot \vec{v}_1 \log\left(\frac{r}{R_\theta}\right) (\hat{n} \cdot \vec{v}_2)^2 + \frac{172}{25} \vec{S}_1 \times \vec{v}_1 \cdot \vec{v}_2 \hat{n} \cdot \vec{v}_2 + \right. \\ & \quad \frac{732}{49} \hat{n} \times \vec{S}_1 \cdot \vec{v}_1 \hat{n} \cdot \vec{v}_1 \hat{n} \cdot \vec{v}_2 - \frac{48}{5} \vec{S}_1 \times \vec{v}_1 \cdot \vec{v}_2 \log\left(\frac{r}{R_\theta}\right) \hat{n} \cdot \vec{v}_2 - \frac{108}{7} \hat{n} \times \vec{S}_1 \cdot \vec{v}_1 \hat{n} \cdot \vec{v}_1 \log\left(\frac{r}{R_\theta}\right) \hat{n} \cdot \vec{v}_2 - \\ & \quad \frac{1644 \vec{S}_1 \times \vec{v}_1 \cdot \vec{v}_2 \hat{n} \cdot \vec{v}_1}{1225} - \frac{1644 \hat{n} \times \vec{S}_1 \cdot \vec{v}_1 \vec{v}_1 \cdot \vec{v}_2}{1225} + \frac{106}{25} \hat{n} \times \vec{S}_1 \cdot \vec{v}_1 \vec{v}_2 \cdot \vec{v}_2 + \frac{108}{35} \vec{S}_1 \times \vec{v}_1 \cdot \vec{v}_2 \hat{n} \cdot \vec{v}_1 \log\left(\frac{r}{R_\theta}\right) + \\ & \quad \frac{108}{35} \hat{n} \times \vec{S}_1 \cdot \vec{v}_1 \vec{v}_1 \cdot \vec{v}_2 \log\left(\frac{r}{R_\theta}\right) - \frac{24}{5} \hat{n} \times \vec{S}_1 \cdot \vec{v}_1 \vec{v}_2 \cdot \vec{v}_2 \log\left(\frac{r}{R_\theta}\right) + \frac{1}{\epsilon_d} \left( -8 \hat{n} \times \vec{S}_1 \cdot \vec{v}_1 (\hat{n} \cdot \vec{v}_2)^2 + \frac{16}{5} \vec{S}_1 \times \vec{v}_1 \cdot \vec{v}_2 \hat{n} \cdot \vec{v}_2 + \right. \\ & \quad \left. \left. \frac{36}{7} \hat{n} \times \vec{S}_1 \cdot \vec{v}_1 \hat{n} \cdot \vec{v}_1 \hat{n} \cdot \vec{v}_2 - \frac{36}{35} \vec{S}_1 \times \vec{v}_1 \cdot \vec{v}_2 \hat{n} \cdot \vec{v}_1 - \frac{36}{35} \hat{n} \times \vec{S}_1 \cdot \vec{v}_1 \vec{v}_1 \cdot \vec{v}_2 + \frac{8}{5} \hat{n} \times \vec{S}_1 \cdot \vec{v}_1 \vec{v}_2 \cdot \vec{v}_2 \right) \right) G^3 \} \end{aligned}$$

{DiagSet[3, 1, 111],

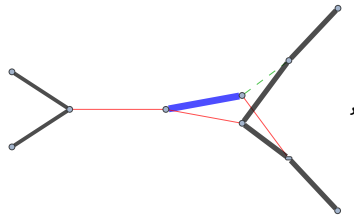

$$\begin{aligned} & \frac{1}{r^3} G^3 m_1^2 m_2 \left( \frac{4 \hat{n} \cdot \vec{a}_1 \hat{n} \times \vec{S}_1 \cdot \vec{v}_1 + 4 \hat{n} \cdot \vec{v}_1 \hat{n} \times \vec{S}_1 \cdot \vec{a}_1 + 4 \hat{n} \cdot \vec{v}_1 \hat{n} \times \vec{S}_1 \cdot \vec{v}_1}{\epsilon_d} - 12 \log\left(\frac{r}{R_\theta}\right) \hat{n} \cdot \vec{a}_1 \hat{n} \times \vec{S}_1 \cdot \vec{v}_1 - 12 \log\left(\frac{r}{R_\theta}\right) \hat{n} \cdot \vec{v}_1 \right. \\ & \quad \left. \hat{n} \times \vec{S}_1 \cdot \vec{a}_1 + 14 \hat{n} \cdot \vec{a}_1 \hat{n} \times \vec{S}_1 \cdot \vec{v}_1 - 2 \hat{n} \cdot \vec{v}_1 \hat{n} \times \vec{S}_1 \cdot \vec{a}_1 - 12 \log\left(\frac{r}{R_\theta}\right) \hat{n} \cdot \vec{v}_1 \hat{n} \times \vec{S}_1 \cdot \vec{v}_1 - 2 \hat{n} \cdot \vec{v}_1 \hat{n} \times \vec{S}_1 \cdot \vec{v}_1 \right) + \\ & \frac{1}{r^4} G^3 m_1^2 m_2 \left( \frac{\frac{8}{5} \vec{v}_1 \cdot \vec{v}_1 \hat{n} \times \vec{S}_1 \cdot \vec{v}_1 - 8 (\hat{n} \cdot \vec{v}_1)^2 \hat{n} \times \vec{S}_1 \cdot \vec{v}_1}{\epsilon_d} + 24 \log\left(\frac{r}{R_\theta}\right) (\hat{n} \cdot \vec{v}_1)^2 \hat{n} \times \vec{S}_1 \cdot \vec{v}_1 - \right. \\ & \quad \left. \frac{24}{5} \log\left(\frac{r}{R_\theta}\right) \vec{v}_1 \cdot \vec{v}_1 \hat{n} \times \vec{S}_1 \cdot \vec{v}_1 - 12 (\hat{n} \cdot \vec{v}_1)^2 \hat{n} \times \vec{S}_1 \cdot \vec{v}_1 + \frac{16}{25} \vec{v}_1 \cdot \vec{v}_1 \hat{n} \times \vec{S}_1 \cdot \vec{v}_1 \right) \} \end{aligned}$$

{DiagSet[3, 1, 112],

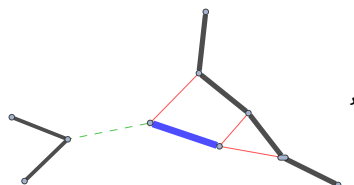

$$\frac{1}{r^3} G^3 m_1^2 m_2 \left( \frac{\frac{4}{5} \vec{S}_1 \times \vec{v}_1 \cdot \vec{a}_2 - \frac{12}{5} \hat{n} \cdot \vec{a}_2 \hat{n} \times \vec{S}_1 \cdot \vec{v}_1}{\epsilon_d} + \frac{36}{5} \log\left(\frac{r}{R_\theta}\right) \hat{n} \cdot \vec{a}_2 \hat{n} \times \vec{S}_1 \cdot \vec{v}_1 - \right. \\ \left. \frac{194}{25} \hat{n} \cdot \vec{a}_2 \hat{n} \times \vec{S}_1 \cdot \vec{v}_1 - \frac{12}{5} \log\left(\frac{r}{R_\theta}\right) \vec{S}_1 \times \vec{v}_1 \cdot \vec{a}_2 + \frac{58}{25} \vec{S}_1 \times \vec{v}_1 \cdot \vec{a}_2 \right) + \frac{1}{r^4} \\ G^3 m_1^2 m_2 \left( \frac{1}{\epsilon_d} \left( -12 (\hat{n} \cdot \vec{v}_2)^2 \hat{n} \times \vec{S}_1 \cdot \vec{v}_1 + \frac{24}{5} \hat{n} \cdot \vec{v}_2 \vec{S}_1 \times \vec{v}_1 \cdot \vec{v}_2 + \frac{20}{7} \hat{n} \cdot \vec{v}_1 \hat{n} \cdot \vec{v}_2 \hat{n} \times \vec{S}_1 \cdot \vec{v}_1 - \right. \right. \\ \left. \frac{4}{7} \hat{n} \cdot \vec{v}_1 \vec{S}_1 \times \vec{v}_1 \cdot \vec{v}_2 - \frac{4}{7} \vec{v}_1 \cdot \vec{v}_2 \hat{n} \times \vec{S}_1 \cdot \vec{v}_1 + \frac{12}{5} \vec{v}_2 \cdot \vec{v}_2 \hat{n} \times \vec{S}_1 \cdot \vec{v}_1 \right) + 36 \log\left(\frac{r}{R_\theta}\right) (\hat{n} \cdot \vec{v}_2)^2 \hat{n} \times \vec{S}_1 \cdot \vec{v}_1 - \\ \frac{72}{5} \log\left(\frac{r}{R_\theta}\right) \hat{n} \cdot \vec{v}_2 \vec{S}_1 \times \vec{v}_1 \cdot \vec{v}_2 - \frac{60}{7} \log\left(\frac{r}{R_\theta}\right) \hat{n} \cdot \vec{v}_1 \hat{n} \cdot \vec{v}_2 \hat{n} \times \vec{S}_1 \cdot \vec{v}_1 + \frac{12}{7} \log\left(\frac{r}{R_\theta}\right) \hat{n} \cdot \vec{v}_1 \vec{S}_1 \times \vec{v}_1 \cdot \vec{v}_2 + \\ \frac{12}{7} \log\left(\frac{r}{R_\theta}\right) \vec{v}_1 \cdot \vec{v}_2 \hat{n} \times \vec{S}_1 \cdot \vec{v}_1 - \frac{36}{5} \log\left(\frac{r}{R_\theta}\right) \vec{v}_2 \cdot \vec{v}_2 \hat{n} \times \vec{S}_1 \cdot \vec{v}_1 - 46 (\hat{n} \cdot \vec{v}_2)^2 \hat{n} \times \vec{S}_1 \cdot \vec{v}_1 + \frac{428}{25} \hat{n} \cdot \vec{v}_2 \vec{S}_1 \times \vec{v}_1 \cdot \vec{v}_2 + \\ \left. \frac{542}{49} \hat{n} \cdot \vec{v}_1 \hat{n} \cdot \vec{v}_2 \hat{n} \times \vec{S}_1 \cdot \vec{v}_1 - \frac{142}{49} \hat{n} \cdot \vec{v}_1 \vec{S}_1 \times \vec{v}_1 \cdot \vec{v}_2 - \frac{318}{245} \vec{v}_1 \cdot \vec{v}_2 \hat{n} \times \vec{S}_1 \cdot \vec{v}_1 + \frac{194}{25} \vec{v}_2 \cdot \vec{v}_2 \hat{n} \times \vec{S}_1 \cdot \vec{v}_1 \right) \Big\}$$

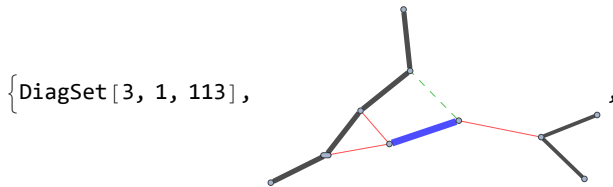

$$\frac{1}{r^3} G^3 m_1^2 m_2 \left( \frac{\frac{12}{5} \hat{n} \cdot \vec{a}_1 \hat{n} \times \vec{S}_1 \cdot \vec{v}_1 - \frac{4}{5} \vec{S}_1 \times \vec{v}_1 \cdot \vec{a}_1}{\epsilon_d} - \frac{36}{5} \log\left(\frac{r}{R_\theta}\right) \hat{n} \cdot \vec{a}_1 \hat{n} \times \vec{S}_1 \cdot \vec{v}_1 + \right. \\ \left. \frac{194}{25} \hat{n} \cdot \vec{a}_1 \hat{n} \times \vec{S}_1 \cdot \vec{v}_1 + \frac{12}{5} \log\left(\frac{r}{R_\theta}\right) \vec{S}_1 \times \vec{v}_1 \cdot \vec{a}_1 - \frac{58}{25} \vec{S}_1 \times \vec{v}_1 \cdot \vec{a}_1 \right) + \frac{1}{r^4} \\ G^3 m_1^2 m_2 \left( \frac{1}{\epsilon_d} \left( -\frac{20}{7} (\hat{n} \cdot \vec{v}_1)^2 \hat{n} \times \vec{S}_1 \cdot \vec{v}_1 - \frac{12}{5} \hat{n} \cdot \vec{v}_1 \vec{S}_1 \times \vec{v}_1 \cdot \vec{v}_2 + 12 \hat{n} \cdot \vec{v}_2 \hat{n} \cdot \vec{v}_1 \hat{n} \times \vec{S}_1 \cdot \vec{v}_1 + \frac{4}{7} \vec{v}_1 \cdot \vec{v}_1 \hat{n} \times \vec{S}_1 \cdot \vec{v}_1 - \right. \right. \\ \left. \frac{12}{5} \vec{v}_1 \cdot \vec{v}_2 \hat{n} \times \vec{S}_1 \cdot \vec{v}_1 \right) + \frac{60}{7} \log\left(\frac{r}{R_\theta}\right) (\hat{n} \cdot \vec{v}_1)^2 \hat{n} \times \vec{S}_1 \cdot \vec{v}_1 + \frac{36}{5} \log\left(\frac{r}{R_\theta}\right) \hat{n} \cdot \vec{v}_1 \vec{S}_1 \times \vec{v}_1 \cdot \vec{v}_2 - 36 \log\left(\frac{r}{R_\theta}\right) \hat{n} \cdot \vec{v}_2 \\ \hat{n} \cdot \vec{v}_1 \hat{n} \times \vec{S}_1 \cdot \vec{v}_1 - \frac{12}{7} \log\left(\frac{r}{R_\theta}\right) \vec{v}_1 \cdot \vec{v}_1 \hat{n} \times \vec{S}_1 \cdot \vec{v}_1 + \frac{36}{5} \log\left(\frac{r}{R_\theta}\right) \vec{v}_1 \cdot \vec{v}_2 \hat{n} \times \vec{S}_1 \cdot \vec{v}_1 - \frac{542}{49} (\hat{n} \cdot \vec{v}_1)^2 \hat{n} \times \vec{S}_1 \cdot \vec{v}_1 - \\ \left. \frac{194}{25} \hat{n} \cdot \vec{v}_1 \vec{S}_1 \times \vec{v}_1 \cdot \vec{v}_2 + 46 \hat{n} \cdot \vec{v}_2 \hat{n} \cdot \vec{v}_1 \hat{n} \times \vec{S}_1 \cdot \vec{v}_1 + \frac{318}{245} \vec{v}_1 \cdot \vec{v}_1 \hat{n} \times \vec{S}_1 \cdot \vec{v}_1 - \frac{194}{25} \vec{v}_1 \cdot \vec{v}_2 \hat{n} \times \vec{S}_1 \cdot \vec{v}_1 \right) \Big\}$$

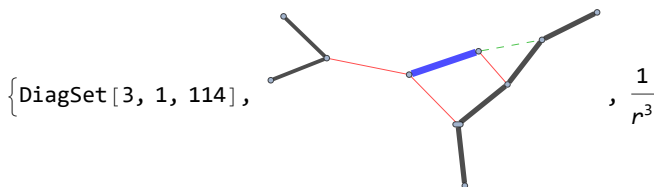

$$G^3 m_1^2 m_2 \left( \frac{24 \hat{n} \cdot \vec{a}_1 \hat{n} \times \vec{S}_1 \cdot \vec{v}_1 - 8 \vec{S}_1 \times \vec{v}_1 \cdot \vec{a}_1}{\epsilon_d} - 72 \log\left(\frac{r}{R_\theta}\right) \hat{n} \cdot \vec{a}_1 \hat{n} \times \vec{S}_1 \cdot \vec{v}_1 + \right. \\ \left. 56 \hat{n} \cdot \vec{a}_1 \hat{n} \times \vec{S}_1 \cdot \vec{v}_1 + 24 \log\left(\frac{r}{R_\theta}\right) \vec{S}_1 \times \vec{v}_1 \cdot \vec{a}_1 - 16 \vec{S}_1 \times \vec{v}_1 \cdot \vec{a}_1 \right) \Big\}$$



{DiagSet[3, 1, 115],

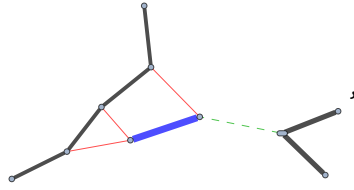

$$\begin{aligned} & \frac{1}{r^2} G^3 \left( -2 \log\left(\frac{r}{R_\theta}\right) \hat{n} \times \vec{a}_1 \cdot \vec{S}_1 + \frac{5}{3} \hat{n} \times \vec{a}_1 \cdot \vec{S}_1 - \frac{5}{3} \hat{n} \times \vec{S}_1 \cdot \vec{v}_1 + \frac{10}{3} \hat{n} \times \vec{a}_1 \cdot \vec{S}_1 + \right. \\ & \quad \left. 2 \hat{n} \times \vec{S}_1 \cdot \vec{v}_1 \log\left(\frac{r}{R_\theta}\right) - 4 \hat{n} \times \vec{a}_1 \cdot \vec{S}_1 \log\left(\frac{r}{R_\theta}\right) + \frac{\frac{2}{3} \hat{n} \times \vec{a}_1 \cdot \vec{S}_1 - \frac{2}{3} \hat{n} \times \vec{S}_1 \cdot \vec{v}_1 + \frac{4}{3} \hat{n} \times \vec{a}_1 \cdot \vec{S}_1}{\epsilon_d} \right) m_2^3 + \\ & \quad \frac{1}{r^3} G^3 \left( -\frac{4}{5} \log\left(\frac{r}{R_\theta}\right) \vec{S}_1 \times \vec{v}_1 \cdot \vec{v}_2 + \frac{23}{75} \vec{S}_1 \times \vec{v}_1 \cdot \vec{v}_2 + \frac{5}{3} \vec{a}_1 \times \vec{S}_1 \cdot \vec{v}_1 - \frac{23}{75} \vec{a}_1 \times \vec{S}_1 \cdot \vec{v}_2 + 7 \hat{n} \times \vec{S}_1 \cdot \vec{v}_1 \hat{n} \cdot \vec{a}_1 + \right. \\ & \quad 14 \hat{n} \times \vec{S}_1 \cdot \vec{v}_1 \hat{n} \cdot \vec{v}_1 - 14 \hat{n} \times \vec{a}_1 \cdot \vec{S}_1 \hat{n} \cdot \vec{v}_1 - \frac{63}{25} \hat{n} \times \vec{S}_1 \cdot \vec{v}_1 \hat{n} \cdot \vec{v}_2 + \frac{17}{25} \hat{n} \times \vec{S}_1 \cdot \vec{v}_2 \hat{n} \cdot \vec{v}_2 + \frac{63}{25} \hat{n} \times \vec{a}_1 \cdot \vec{S}_1 \hat{n} \cdot \vec{v}_2 - \\ & \quad 2 \vec{a}_1 \times \vec{S}_1 \cdot \vec{v}_1 \log\left(\frac{r}{R_\theta}\right) + \frac{4}{5} \vec{a}_1 \times \vec{S}_1 \cdot \vec{v}_2 \log\left(\frac{r}{R_\theta}\right) - 6 \hat{n} \times \vec{S}_1 \cdot \vec{v}_1 \hat{n} \cdot \vec{a}_1 \log\left(\frac{r}{R_\theta}\right) - 12 \hat{n} \times \vec{S}_1 \cdot \vec{v}_1 \hat{n} \cdot \vec{v}_1 \log\left(\frac{r}{R_\theta}\right) + \\ & \quad 12 \hat{n} \times \vec{a}_1 \cdot \vec{S}_1 \hat{n} \cdot \vec{v}_1 \log\left(\frac{r}{R_\theta}\right) + \frac{12}{5} \hat{n} \times \vec{S}_1 \cdot \vec{v}_1 \hat{n} \cdot \vec{v}_2 \log\left(\frac{r}{R_\theta}\right) - \frac{3}{5} \hat{n} \times \vec{S}_1 \cdot \vec{v}_2 \hat{n} \cdot \vec{v}_2 \log\left(\frac{r}{R_\theta}\right) - \\ & \quad \frac{12}{5} \hat{n} \times \vec{a}_1 \cdot \vec{S}_1 \hat{n} \cdot \vec{v}_2 \log\left(\frac{r}{R_\theta}\right) + \frac{1}{\epsilon_d} \left( \frac{4}{15} \vec{S}_1 \times \vec{v}_1 \cdot \vec{v}_2 + \frac{2}{3} \vec{a}_1 \times \vec{S}_1 \cdot \vec{v}_1 - \frac{4}{15} \vec{a}_1 \times \vec{S}_1 \cdot \vec{v}_2 + 2 \hat{n} \times \vec{S}_1 \cdot \vec{v}_1 \hat{n} \cdot \vec{a}_1 + \right. \\ & \quad \left. 4 \hat{n} \times \vec{S}_1 \cdot \vec{v}_1 \hat{n} \cdot \vec{v}_1 - 4 \hat{n} \times \vec{a}_1 \cdot \vec{S}_1 \hat{n} \cdot \vec{v}_1 - \frac{4}{5} \hat{n} \times \vec{S}_1 \cdot \vec{v}_1 \hat{n} \cdot \vec{v}_2 + \frac{1}{5} \hat{n} \times \vec{S}_1 \cdot \vec{v}_2 \hat{n} \cdot \vec{v}_2 + \frac{4}{5} \hat{n} \times \vec{a}_1 \cdot \vec{S}_1 \hat{n} \cdot \vec{v}_2 \right) \left. \right) m_2^3 + \frac{1}{r^4} \\ & \quad G^3 \left( -41 \hat{n} \times \vec{S}_1 \cdot \vec{v}_1 (\hat{n} \cdot \vec{v}_1)^2 + 30 \hat{n} \times \vec{S}_1 \cdot \vec{v}_1 \log\left(\frac{r}{R_\theta}\right) (\hat{n} \cdot \vec{v}_1)^2 - \frac{58}{25} \vec{S}_1 \times \vec{v}_1 \cdot \vec{v}_2 \hat{n} \cdot \vec{v}_1 + 15 \hat{n} \times \vec{S}_1 \cdot \vec{v}_1 \hat{n} \cdot \vec{v}_2 \hat{n} \cdot \vec{v}_1 - \right. \\ & \quad 4 \hat{n} \times \vec{S}_1 \cdot \vec{v}_2 \hat{n} \cdot \vec{v}_2 \hat{n} \cdot \vec{v}_1 + \frac{12}{5} \vec{S}_1 \times \vec{v}_1 \cdot \vec{v}_2 \log\left(\frac{r}{R_\theta}\right) \hat{n} \cdot \vec{v}_1 - 12 \hat{n} \times \vec{S}_1 \cdot \vec{v}_1 \hat{n} \cdot \vec{v}_2 \log\left(\frac{r}{R_\theta}\right) \hat{n} \cdot \vec{v}_1 + \\ & \quad 3 \hat{n} \times \vec{S}_1 \cdot \vec{v}_2 \hat{n} \cdot \vec{v}_2 \log\left(\frac{r}{R_\theta}\right) \hat{n} \cdot \vec{v}_1 - \frac{17}{25} \vec{S}_1 \times \vec{v}_1 \cdot \vec{v}_2 \hat{n} \cdot \vec{v}_2 + 7 \hat{n} \times \vec{S}_1 \cdot \vec{v}_1 \vec{v}_1 \cdot \vec{v}_1 - \\ & \quad \frac{48}{25} \hat{n} \times \vec{S}_1 \cdot \vec{v}_1 \vec{v}_1 \cdot \vec{v}_2 + \frac{17}{25} \hat{n} \times \vec{S}_1 \cdot \vec{v}_2 \vec{v}_1 \cdot \vec{v}_2 + \frac{9}{5} \hat{n} \times \vec{S}_1 \cdot \vec{v}_2 \vec{v}_2 \cdot \vec{v}_2 + \frac{3}{5} \vec{S}_1 \times \vec{v}_1 \cdot \vec{v}_2 \hat{n} \cdot \vec{v}_2 \log\left(\frac{r}{R_\theta}\right) - \\ & \quad 6 \hat{n} \times \vec{S}_1 \cdot \vec{v}_1 \vec{v}_1 \cdot \vec{v}_1 \log\left(\frac{r}{R_\theta}\right) + \frac{12}{5} \hat{n} \times \vec{S}_1 \cdot \vec{v}_1 \vec{v}_1 \cdot \vec{v}_2 \log\left(\frac{r}{R_\theta}\right) - \frac{3}{5} \hat{n} \times \vec{S}_1 \cdot \vec{v}_2 \vec{v}_1 \cdot \vec{v}_2 \log\left(\frac{r}{R_\theta}\right) + \frac{1}{\epsilon_d} \\ & \quad \left( -10 \hat{n} \times \vec{S}_1 \cdot \vec{v}_1 (\hat{n} \cdot \vec{v}_1)^2 - \frac{4}{5} \vec{S}_1 \times \vec{v}_1 \cdot \vec{v}_2 \hat{n} \cdot \vec{v}_1 + 4 \hat{n} \times \vec{S}_1 \cdot \vec{v}_1 \hat{n} \cdot \vec{v}_2 \hat{n} \cdot \vec{v}_1 - \hat{n} \times \vec{S}_1 \cdot \vec{v}_2 \hat{n} \cdot \vec{v}_2 \hat{n} \cdot \vec{v}_1 - \right. \\ & \quad \left. \frac{1}{5} \vec{S}_1 \times \vec{v}_1 \cdot \vec{v}_2 \hat{n} \cdot \vec{v}_2 + 2 \hat{n} \times \vec{S}_1 \cdot \vec{v}_1 \vec{v}_1 \cdot \vec{v}_1 - \frac{4}{5} \hat{n} \times \vec{S}_1 \cdot \vec{v}_1 \vec{v}_1 \cdot \vec{v}_2 + \frac{1}{5} \hat{n} \times \vec{S}_1 \cdot \vec{v}_2 \vec{v}_1 \cdot \vec{v}_2 \right) \left. \right) m_2^3 \Big\} \end{aligned}$$

{DiagSet[3, 1, 116],

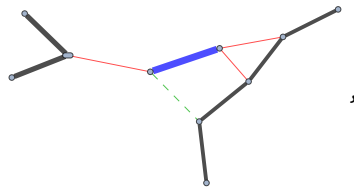

$$\begin{aligned} & \frac{1}{r^3} G^3 \left( -4 \log\left(\frac{r}{R_\theta}\right) \vec{S}_1 \times \vec{v}_1 \cdot \vec{v}_2 + \frac{8}{3} \vec{S}_1 \times \vec{v}_1 \cdot \vec{v}_2 - \frac{8}{3} \vec{a}_1 \times \vec{S}_1 \cdot \vec{v}_2 + \frac{8}{3} \vec{a}_2 \times \vec{S}_1 \cdot \vec{v}_1 - 12 \hat{n} \times \vec{S}_1 \cdot \vec{v}_1 \hat{n} \cdot \vec{a}_2 - \right. \\ & \quad \left. 12 \hat{n} \times \vec{S}_1 \cdot \vec{v}_1 \hat{n} \cdot \vec{v}_2 + 12 \hat{n} \times \vec{a}_1 \cdot \vec{S}_1 \hat{n} \cdot \vec{v}_2 + 4 \vec{a}_1 \times \vec{S}_1 \cdot \vec{v}_2 \log\left(\frac{r}{R_\theta}\right) - 4 \vec{a}_2 \times \vec{S}_1 \cdot \vec{v}_1 \log\left(\frac{r}{R_\theta}\right) + \right. \end{aligned}$$

$$\begin{aligned}
& 12 \hat{n} \times \vec{S}_1 \cdot \vec{v}_1 \hat{n} \cdot \vec{a}_2 \log\left(\frac{r}{R_\theta}\right) + 12 \hat{n} \times \vec{S}_1 \cdot \vec{v}_1 \hat{n} \cdot \vec{v}_2 \log\left(\frac{r}{R_\theta}\right) - 12 \hat{n} \times \vec{a}_1 \cdot \vec{S}_1 \hat{n} \cdot \vec{v}_2 \log\left(\frac{r}{R_\theta}\right) + \frac{1}{\epsilon_d} \\
& \left( \frac{4}{3} \vec{S}_1 \times \vec{v}_1 \cdot \vec{v}_2 - \frac{4}{3} \vec{a}_1 \times \vec{S}_1 \cdot \vec{v}_2 + \frac{4}{3} \vec{a}_2 \times \vec{S}_1 \cdot \vec{v}_1 - 4 \hat{n} \times \vec{S}_1 \cdot \vec{v}_1 \hat{n} \cdot \vec{a}_2 - 4 \hat{n} \times \vec{S}_1 \cdot \vec{v}_1 \hat{n} \cdot \vec{v}_2 + 4 \hat{n} \times \vec{a}_1 \cdot \vec{S}_1 \hat{n} \cdot \vec{v}_2 \right) m_2^3 + \\
& \frac{1}{r^4} G^3 \left( -26 \hat{n} \times \vec{S}_1 \cdot \vec{v}_1 (\hat{n} \cdot \vec{v}_2)^2 + 24 \hat{n} \times \vec{S}_1 \cdot \vec{v}_1 \log\left(\frac{r}{R_\theta}\right) (\hat{n} \cdot \vec{v}_2)^2 + \frac{212}{25} \vec{S}_1 \times \vec{v}_1 \cdot \vec{v}_2 \hat{n} \cdot \vec{v}_2 + \right. \\
& 72 \hat{n} \times \vec{S}_1 \cdot \vec{v}_1 \hat{n} \cdot \vec{v}_1 \hat{n} \cdot \vec{v}_2 - \frac{48}{5} \vec{S}_1 \times \vec{v}_1 \cdot \vec{v}_2 \log\left(\frac{r}{R_\theta}\right) \hat{n} \cdot \vec{v}_2 - 60 \hat{n} \times \vec{S}_1 \cdot \vec{v}_1 \hat{n} \cdot \vec{v}_1 \log\left(\frac{r}{R_\theta}\right) \hat{n} \cdot \vec{v}_2 - \\
& 12 \vec{S}_1 \times \vec{v}_1 \cdot \vec{v}_2 \hat{n} \cdot \vec{v}_1 - 12 \hat{n} \times \vec{S}_1 \cdot \vec{v}_1 \vec{v}_1 \cdot \vec{v}_2 + \frac{66}{25} \hat{n} \times \vec{S}_1 \cdot \vec{v}_1 \vec{v}_2 \cdot \vec{v}_2 + 12 \vec{S}_1 \times \vec{v}_1 \cdot \vec{v}_2 \hat{n} \cdot \vec{v}_1 \log\left(\frac{r}{R_\theta}\right) + \\
& 12 \hat{n} \times \vec{S}_1 \cdot \vec{v}_1 \vec{v}_1 \cdot \vec{v}_2 \log\left(\frac{r}{R_\theta}\right) - \frac{24}{5} \hat{n} \times \vec{S}_1 \cdot \vec{v}_1 \vec{v}_2 \cdot \vec{v}_2 \log\left(\frac{r}{R_\theta}\right) + \frac{1}{\epsilon_d} \left( -8 \hat{n} \times \vec{S}_1 \cdot \vec{v}_1 (\hat{n} \cdot \vec{v}_2)^2 + \frac{16}{5} \vec{S}_1 \times \vec{v}_1 \cdot \vec{v}_2 \hat{n} \cdot \vec{v}_2 + \right. \\
& \left. \left. 20 \hat{n} \times \vec{S}_1 \cdot \vec{v}_1 \hat{n} \cdot \vec{v}_1 \hat{n} \cdot \vec{v}_2 - 4 \vec{S}_1 \times \vec{v}_1 \cdot \vec{v}_2 \hat{n} \cdot \vec{v}_1 - 4 \hat{n} \times \vec{S}_1 \cdot \vec{v}_1 \vec{v}_1 \cdot \vec{v}_2 + \frac{8}{5} \hat{n} \times \vec{S}_1 \cdot \vec{v}_1 \vec{v}_2 \cdot \vec{v}_2 \right) m_2^3 \right\}
\end{aligned}$$

$$\left\{ \text{DiagSet}[3, 1, 117], \right.$$
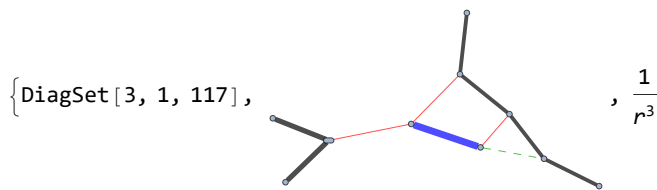

$$, \frac{1}{r^3}$$

$$\begin{aligned}
& G^3 m_2^3 \left( \frac{8 \vec{a}_2 \times \vec{S}_1 \cdot \vec{v}_1 - 24 \hat{n} \cdot \vec{a}_2 \hat{n} \times \vec{S}_1 \cdot \vec{v}_1}{\epsilon_d} + 72 \log\left(\frac{r}{R_\theta}\right) \hat{n} \cdot \vec{a}_2 \hat{n} \times \vec{S}_1 \cdot \vec{v}_1 - \right. \\
& \left. 72 \hat{n} \cdot \vec{a}_2 \hat{n} \times \vec{S}_1 \cdot \vec{v}_1 - 24 \log\left(\frac{r}{R_\theta}\right) \vec{a}_2 \times \vec{S}_1 \cdot \vec{v}_1 + 16 \vec{a}_2 \times \vec{S}_1 \cdot \vec{v}_1 \right\}
\end{aligned}$$

$$\left\{ \text{DiagSet}[3, 1, 118], \right.$$
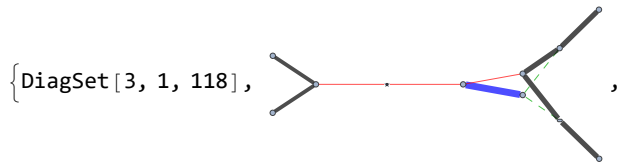

$$,$$

$$\begin{aligned}
& \frac{1}{r^3} G^3 m_1^2 m_2 \left( \frac{\hat{n} \cdot \vec{v}_2 \hat{n} \times \vec{S}_1 \cdot \vec{a}_1 - \frac{1}{3} \vec{S}_1 \times \vec{a}_1 \cdot \vec{v}_2 + \hat{n} \cdot \vec{v}_2 \hat{n} \times \vec{S}_1 \cdot \vec{v}_1 - \frac{1}{3} \vec{S}_1 \times \vec{v}_1 \cdot \vec{v}_2}{\epsilon_d} - \right. \\
& 3 \log\left(\frac{r}{R_\theta}\right) \hat{n} \cdot \vec{v}_2 \hat{n} \times \vec{S}_1 \cdot \vec{a}_1 + \frac{11}{5} \hat{n} \cdot \vec{v}_2 \hat{n} \times \vec{S}_1 \cdot \vec{a}_1 + \log\left(\frac{r}{R_\theta}\right) \vec{S}_1 \times \vec{a}_1 \cdot \vec{v}_2 - \frac{2}{5} \vec{S}_1 \times \vec{a}_1 \cdot \vec{v}_2 - \\
& \left. 3 \log\left(\frac{r}{R_\theta}\right) \hat{n} \cdot \vec{v}_2 \hat{n} \times \vec{S}_1 \cdot \vec{v}_1 + \frac{11}{5} \hat{n} \cdot \vec{v}_2 \hat{n} \times \vec{S}_1 \cdot \vec{v}_1 + \log\left(\frac{r}{R_\theta}\right) \frac{1}{\vec{S}_1 \times \vec{v}_1 \cdot \vec{v}_2} - \frac{2}{5} \frac{1}{\vec{S}_1 \times \vec{v}_1 \cdot \vec{v}_2} \right) + \frac{1}{r^4} \\
& G^3 m_1^2 m_2 \left( \frac{\hat{n} \cdot \vec{v}_1 \vec{S}_1 \times \vec{v}_1 \cdot \vec{v}_2 - 5 \hat{n} \cdot \vec{v}_2 \hat{n} \cdot \vec{v}_1 \hat{n} \times \vec{S}_1 \cdot \vec{v}_1 + \vec{v}_1 \cdot \vec{v}_2 \hat{n} \times \vec{S}_1 \cdot \vec{v}_1}{\epsilon_d} - 3 \log\left(\frac{r}{R_\theta}\right) \hat{n} \cdot \vec{v}_1 \vec{S}_1 \times \vec{v}_1 \cdot \vec{v}_2 + \right. \\
& 15 \log\left(\frac{r}{R_\theta}\right) \hat{n} \cdot \vec{v}_2 \hat{n} \cdot \vec{v}_1 \hat{n} \times \vec{S}_1 \cdot \vec{v}_1 - 3 \log\left(\frac{r}{R_\theta}\right) \vec{v}_1 \cdot \vec{v}_2 \hat{n} \times \vec{S}_1 \cdot \vec{v}_1 + \\
& \left. \frac{11}{5} \hat{n} \cdot \vec{v}_1 \vec{S}_1 \times \vec{v}_1 \cdot \vec{v}_2 - 14 \hat{n} \cdot \vec{v}_2 \hat{n} \cdot \vec{v}_1 \hat{n} \times \vec{S}_1 \cdot \vec{v}_1 + \frac{11}{5} \vec{v}_1 \cdot \vec{v}_2 \hat{n} \times \vec{S}_1 \cdot \vec{v}_1 \right\}
\end{aligned}$$

$$\left\{ \text{DiagSet}[3, 1, 119], \right.$$
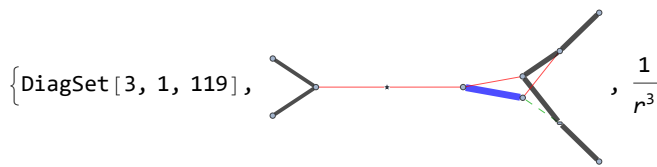

$$, \frac{1}{r^3}$$

$$G^3 m_1^2 m_2 \left( \frac{-\frac{1}{2} \hat{n} \cdot \vec{v}_2 \hat{n} \times \vec{S}_1 \cdot \vec{a}_1 + \frac{1}{6} \vec{S}_1 \times \vec{a}_1 \cdot \vec{v}_2 - \frac{1}{2} \hat{n} \cdot \vec{v}_2 \hat{n} \times \vec{S}_1 \cdot \vec{v}_1 + \frac{1}{6} \vec{S}_1 \times \vec{v}_1 \cdot \vec{v}_2}{\epsilon_d} + \frac{3}{2} \log\left(\frac{r}{R_\theta}\right) \hat{n} \cdot \vec{v}_2 \hat{n} \times \vec{S}_1 \cdot \vec{a}_1 - \frac{1}{2} \hat{n} \cdot \vec{v}_2 \right.$$

$$\left. \hat{n} \times \vec{S}_1 \cdot \vec{a}_1 - \frac{1}{2} \log\left(\frac{r}{R_\theta}\right) \vec{S}_1 \times \vec{a}_1 \cdot \vec{v}_2 + \frac{3}{2} \log\left(\frac{r}{R_\theta}\right) \hat{n} \cdot \vec{v}_2 \hat{n} \times \vec{S}_1 \cdot \vec{v}_1 - \frac{1}{2} \hat{n} \cdot \vec{v}_2 \hat{n} \times \vec{S}_1 \cdot \vec{v}_1 - \frac{1}{2} \log\left(\frac{r}{R_\theta}\right) \vec{S}_1 \times \vec{v}_1 \cdot \vec{v}_2 \right) +$$

$$\frac{1}{r^4} G^3 m_1^2 m_2 \left( \frac{-\frac{1}{2} \hat{n} \cdot \vec{v}_1 \vec{S}_1 \times \vec{v}_1 \cdot \vec{v}_2 + \frac{5}{2} \hat{n} \cdot \vec{v}_2 \hat{n} \cdot \vec{v}_1 \hat{n} \times \vec{S}_1 \cdot \vec{v}_1 - \frac{1}{2} \vec{v}_1 \cdot \vec{v}_2 \hat{n} \times \vec{S}_1 \cdot \vec{v}_1}{\epsilon_d} + \frac{3}{2} \log\left(\frac{r}{R_\theta}\right) \hat{n} \cdot \vec{v}_1 \vec{S}_1 \times \vec{v}_1 \cdot \vec{v}_2 -$$

$$\frac{15}{2} \log\left(\frac{r}{R_\theta}\right) \hat{n} \cdot \vec{v}_2 \hat{n} \cdot \vec{v}_1 \hat{n} \times \vec{S}_1 \cdot \vec{v}_1 + \frac{3}{2} \log\left(\frac{r}{R_\theta}\right) \vec{v}_1 \cdot \vec{v}_2 \hat{n} \times \vec{S}_1 \cdot \vec{v}_1 -$$

$$\left. \frac{1}{2} \hat{n} \cdot \vec{v}_1 \vec{S}_1 \times \vec{v}_1 \cdot \vec{v}_2 + 4 \hat{n} \cdot \vec{v}_2 \hat{n} \cdot \vec{v}_1 \hat{n} \times \vec{S}_1 \cdot \vec{v}_1 - \frac{1}{2} \vec{v}_1 \cdot \vec{v}_2 \hat{n} \times \vec{S}_1 \cdot \vec{v}_1 \right) \Bigg\}$$

$$\left\{ \text{DiagSet}[3, 1, 120], \right.$$
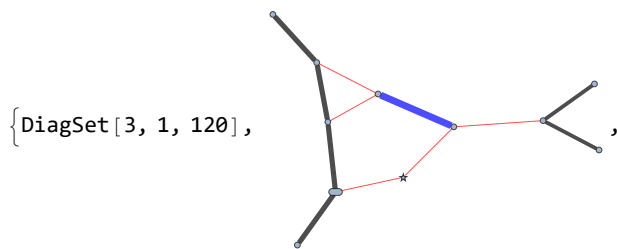

$$,$$

$$\frac{1}{r^3} G^3 m_1^2 m_2 \left( \frac{\frac{1}{5} \hat{n} \cdot \vec{v}_1 \hat{n} \times \vec{S}_1 \cdot \vec{a}_1 + \frac{1}{15} \vec{S}_1 \times \vec{v}_1 \cdot \vec{a}_1 + \frac{1}{5} \hat{n} \cdot \vec{v}_1 \hat{n} \times \vec{S}_1 \cdot \vec{v}_1}{\epsilon_d} - \frac{3}{5} \log\left(\frac{r}{R_\theta}\right) \hat{n} \cdot \vec{v}_1 \hat{n} \times \vec{S}_1 \cdot \vec{a}_1 +$$

$$\frac{7}{25} \hat{n} \cdot \vec{v}_1 \hat{n} \times \vec{S}_1 \cdot \vec{a}_1 + \hat{n} \cdot \vec{v}_2 \hat{n} \times \vec{S}_1 \cdot \vec{a}_1 - \frac{1}{5} \log\left(\frac{r}{R_\theta}\right) \vec{S}_1 \times \vec{v}_1 \cdot \vec{a}_1 - \frac{1}{3} \vec{S}_1 \times \vec{a}_1 \cdot \vec{v}_2 + \frac{22}{75} \vec{S}_1 \times \vec{v}_1 \cdot \vec{a}_1 -$$

$$\left. \frac{3}{5} \log\left(\frac{r}{R_\theta}\right) \hat{n} \cdot \vec{v}_1 \hat{n} \times \vec{S}_1 \cdot \vec{v}_1 + \frac{7}{25} \hat{n} \cdot \vec{v}_1 \hat{n} \times \vec{S}_1 \cdot \vec{v}_1 + \hat{n} \cdot \vec{v}_2 \hat{n} \times \vec{S}_1 \cdot \vec{v}_1 - \frac{1}{3} \vec{S}_1 \times \vec{v}_1 \cdot \vec{v}_2 \right) + \frac{1}{r^4} G^3 m_1^2 m_2 \left( \frac{1}{\epsilon_d} \right.$$

$$\left( -\frac{2}{7} (\hat{n} \cdot \vec{v}_1)^2 \hat{n} \times \vec{S}_1 \cdot \vec{v}_1 + \frac{1}{5} \hat{n} \cdot \vec{v}_1 \vec{S}_1 \times \vec{v}_1 \cdot \vec{v}_2 - \hat{n} \cdot \vec{v}_2 \hat{n} \cdot \vec{v}_1 \hat{n} \times \vec{S}_1 \cdot \vec{v}_1 + \frac{2}{35} \vec{v}_1 \cdot \vec{v}_1 \hat{n} \times \vec{S}_1 \cdot \vec{v}_1 + \frac{1}{5} \vec{v}_1 \cdot \vec{v}_2 \hat{n} \times \vec{S}_1 \cdot \vec{v}_1 \right) +$$

$$\frac{6}{7} \log\left(\frac{r}{R_\theta}\right) (\hat{n} \cdot \vec{v}_1)^2 \hat{n} \times \vec{S}_1 \cdot \vec{v}_1 - \frac{3}{5} \log\left(\frac{r}{R_\theta}\right) \hat{n} \cdot \vec{v}_1 \vec{S}_1 \times \vec{v}_1 \cdot \vec{v}_2 + 3 \log\left(\frac{r}{R_\theta}\right) \hat{n} \cdot \vec{v}_2 \hat{n} \cdot \vec{v}_1 \hat{n} \times \vec{S}_1 \cdot \vec{v}_1 -$$

$$\frac{6}{35} \log\left(\frac{r}{R_\theta}\right) \vec{v}_1 \cdot \vec{v}_1 \hat{n} \times \vec{S}_1 \cdot \vec{v}_1 - \frac{3}{5} \log\left(\frac{r}{R_\theta}\right) \vec{v}_1 \cdot \vec{v}_2 \hat{n} \times \vec{S}_1 \cdot \vec{v}_1 - \frac{8}{49} (\hat{n} \cdot \vec{v}_1)^2 \hat{n} \times \vec{S}_1 \cdot \vec{v}_1 +$$

$$\left. \frac{32}{25} \hat{n} \cdot \vec{v}_1 \vec{S}_1 \times \vec{v}_1 \cdot \vec{v}_2 - 7 \hat{n} \cdot \vec{v}_2 \hat{n} \cdot \vec{v}_1 \hat{n} \times \vec{S}_1 \cdot \vec{v}_1 + \frac{418 \vec{v}_1 \cdot \vec{v}_1 \hat{n} \times \vec{S}_1 \cdot \vec{v}_1}{1225} + \frac{32}{25} \vec{v}_1 \cdot \vec{v}_2 \hat{n} \times \vec{S}_1 \cdot \vec{v}_1 \right) \Bigg\}$$

{DiagSet[3, 1, 121],

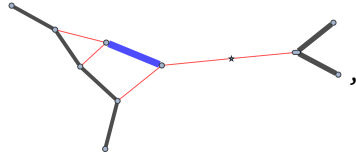

$$\frac{1}{r^3} G^3 m_2^3 \left( \frac{\hat{n} \cdot \vec{v}_2 \hat{n} \times \vec{a}_1 \cdot \vec{S}_1 - \frac{1}{3} \vec{a}_1 \times \vec{S}_1 \cdot \vec{v}_2 - \hat{n} \cdot \vec{v}_2 \hat{n} \times \vec{S}_1 \cdot \vec{v}_1 + \frac{1}{3} \vec{S}_1 \times \vec{v}_1 \cdot \vec{v}_2}{\epsilon_d} - \right.$$

$$3 \log \left( \frac{r}{R_\theta} \right) \hat{n} \cdot \vec{v}_2 \hat{n} \times \vec{a}_1 \cdot \vec{S}_1 + \frac{7}{2} \hat{n} \cdot \vec{v}_2 \hat{n} \times \vec{a}_1 \cdot \vec{S}_1 + \log \left( \frac{r}{R_\theta} \right) \vec{a}_1 \times \vec{S}_1 \cdot \vec{v}_2 - \frac{5}{6} \vec{a}_1 \times \vec{S}_1 \cdot \vec{v}_2 +$$

$$3 \log \left( \frac{r}{R_\theta} \right) \hat{n} \cdot \vec{v}_2 \hat{n} \times \vec{S}_1 \cdot \vec{v}_1 - \frac{7}{2} \hat{n} \cdot \vec{v}_2 \hat{n} \times \vec{S}_1 \cdot \vec{v}_1 - \log \left( \frac{r}{R_\theta} \right) \vec{S}_1 \times \vec{v}_1 \cdot \vec{v}_2 + \frac{5}{6} \vec{S}_1 \times \vec{v}_1 \cdot \vec{v}_2 \left. \right) + \frac{1}{r^4}$$

$$G^3 m_2^3 \left( \frac{\hat{n} \cdot \vec{v}_1 \left( - \left( \vec{S}_1 \times \vec{v}_1 \cdot \vec{v}_2 \right) \right) + 5 \hat{n} \cdot \vec{v}_2 \hat{n} \cdot \vec{v}_1 \hat{n} \times \vec{S}_1 \cdot \vec{v}_1 - \vec{v}_1 \cdot \vec{v}_2 \hat{n} \times \vec{S}_1 \cdot \vec{v}_1}{\epsilon_d} + 3 \log \left( \frac{r}{R_\theta} \right) \hat{n} \cdot \vec{v}_1 \vec{S}_1 \times \vec{v}_1 \cdot \vec{v}_2 - \right.$$

$$15 \log \left( \frac{r}{R_\theta} \right) \hat{n} \cdot \vec{v}_2 \hat{n} \cdot \vec{v}_1 \hat{n} \times \vec{S}_1 \cdot \vec{v}_1 + 3 \log \left( \frac{r}{R_\theta} \right) \vec{v}_1 \cdot \vec{v}_2 \hat{n} \times \vec{S}_1 \cdot \vec{v}_1 -$$

$$\left. \frac{7}{2} \hat{n} \cdot \vec{v}_1 \vec{S}_1 \times \vec{v}_1 \cdot \vec{v}_2 + \frac{41}{2} \hat{n} \cdot \vec{v}_2 \hat{n} \cdot \vec{v}_1 \hat{n} \times \vec{S}_1 \cdot \vec{v}_1 - \frac{7}{2} \vec{v}_1 \cdot \vec{v}_2 \hat{n} \times \vec{S}_1 \cdot \vec{v}_1 \right\}$$

{DiagSet[3, 1, 122],

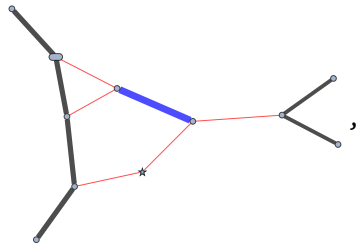

$$\frac{1}{r^3} G^3 m_1^2 m_2 \left( \frac{\frac{1}{5} \hat{n} \cdot \vec{v}_1 \hat{n} \times \vec{S}_1 \cdot \vec{a}_1 + \frac{1}{15} \vec{S}_1 \times \vec{v}_1 \cdot \vec{a}_1 + \frac{1}{5} \hat{n} \cdot \vec{v}_1 \hat{n} \times \vec{S}_1 \cdot \vec{v}_1}{\epsilon_d} - \frac{3}{5} \log \left( \frac{r}{R_\theta} \right) \hat{n} \cdot \vec{v}_1 \hat{n} \times \vec{S}_1 \cdot \vec{a}_1 + \frac{7}{25} \hat{n} \cdot \vec{v}_1 \hat{n} \times \vec{S}_1 \cdot \vec{a}_1 - \right.$$

$$\left. \frac{1}{5} \log \left( \frac{r}{R_\theta} \right) \vec{S}_1 \times \vec{v}_1 \cdot \vec{a}_1 + \frac{22}{75} \vec{S}_1 \times \vec{v}_1 \cdot \vec{a}_1 - \frac{3}{5} \log \left( \frac{r}{R_\theta} \right) \hat{n} \cdot \vec{v}_1 \hat{n} \times \vec{S}_1 \cdot \vec{v}_1 + \frac{7}{25} \hat{n} \cdot \vec{v}_1 \hat{n} \times \vec{S}_1 \cdot \vec{v}_1 \right) + \frac{1}{r^4} G^3 m_1^2 m_2$$

$$\left( \frac{1}{\epsilon_d} \left( -\frac{5}{7} (\hat{n} \cdot \vec{v}_1)^2 \hat{n} \times \vec{S}_1 \cdot \vec{v}_1 - \frac{1}{5} \hat{n} \cdot \vec{v}_1 \vec{S}_1 \times \vec{v}_1 \cdot \vec{v}_2 + \hat{n} \cdot \vec{v}_2 \hat{n} \cdot \vec{v}_1 \hat{n} \times \vec{S}_1 \cdot \vec{v}_1 + \frac{1}{7} \vec{v}_1 \cdot \vec{v}_1 \hat{n} \times \vec{S}_1 \cdot \vec{v}_1 - \frac{1}{5} \vec{v}_1 \cdot \vec{v}_2 \hat{n} \times \vec{S}_1 \cdot \vec{v}_1 \right) + \right.$$

$$\frac{15}{7} \log \left( \frac{r}{R_\theta} \right) (\hat{n} \cdot \vec{v}_1)^2 \hat{n} \times \vec{S}_1 \cdot \vec{v}_1 + \frac{3}{5} \log \left( \frac{r}{R_\theta} \right) \hat{n} \cdot \vec{v}_1 \vec{S}_1 \times \vec{v}_1 \cdot \vec{v}_2 - 3 \log \left( \frac{r}{R_\theta} \right) \hat{n} \cdot \vec{v}_2 \hat{n} \cdot \vec{v}_1 \hat{n} \times \vec{S}_1 \cdot \vec{v}_1 -$$

$$\frac{3}{7} \log \left( \frac{r}{R_\theta} \right) \vec{v}_1 \cdot \vec{v}_1 \hat{n} \times \vec{S}_1 \cdot \vec{v}_1 + \frac{3}{5} \log \left( \frac{r}{R_\theta} \right) \vec{v}_1 \cdot \vec{v}_2 \hat{n} \times \vec{S}_1 \cdot \vec{v}_1 - \frac{9\theta}{49} (\hat{n} \cdot \vec{v}_1)^2 \hat{n} \times \vec{S}_1 \cdot \vec{v}_1 -$$

$$\left. \frac{7}{25} \hat{n} \cdot \vec{v}_1 \vec{S}_1 \times \vec{v}_1 \cdot \vec{v}_2 + 2 \hat{n} \cdot \vec{v}_2 \hat{n} \cdot \vec{v}_1 \hat{n} \times \vec{S}_1 \cdot \vec{v}_1 + \frac{181}{245} \vec{v}_1 \cdot \vec{v}_1 \hat{n} \times \vec{S}_1 \cdot \vec{v}_1 - \frac{7}{25} \vec{v}_1 \cdot \vec{v}_2 \hat{n} \times \vec{S}_1 \cdot \vec{v}_1 \right\}$$

{DiagSet[3, 1, 123],

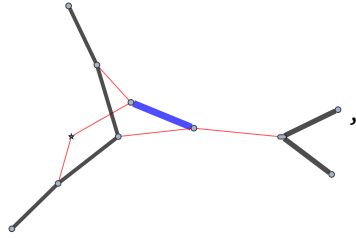

$$\frac{1}{r^3} G^3 \left( -2 \log \left( \frac{r}{R_0} \right) \frac{1}{S_1} \times \vec{v}_1 \cdot \vec{v}_2 + \frac{13}{9} \frac{1}{S_1} \times \vec{v}_1 \cdot \vec{v}_2 - \frac{13}{9} \vec{a}_1 \times \vec{S}_1 \cdot \vec{v}_2 - \right. \\ \left. \frac{19}{3} \hat{n} \times \vec{S}_1 \cdot \vec{v}_1 \hat{n} \cdot \vec{v}_2 + \frac{19}{3} \hat{n} \times \vec{a}_1 \cdot \vec{S}_1 \hat{n} \cdot \vec{v}_2 + 2 \vec{a}_1 \times \vec{S}_1 \cdot \vec{v}_2 \log \left( \frac{r}{R_0} \right) + 6 \hat{n} \times \vec{S}_1 \cdot \vec{v}_1 \hat{n} \cdot \vec{v}_2 \log \left( \frac{r}{R_0} \right) - \right. \\ \left. 6 \hat{n} \times \vec{a}_1 \cdot \vec{S}_1 \hat{n} \cdot \vec{v}_2 \log \left( \frac{r}{R_0} \right) + \frac{\frac{2}{3} \frac{1}{S_1} \times \vec{v}_1 \cdot \vec{v}_2 - \frac{2}{3} \vec{a}_1 \times \vec{S}_1 \cdot \vec{v}_2 - 2 \hat{n} \times \vec{S}_1 \cdot \vec{v}_1 \hat{n} \cdot \vec{v}_2 + 2 \hat{n} \times \vec{a}_1 \cdot \vec{S}_1 \hat{n} \cdot \vec{v}_2}{\epsilon_d} \right) m_2^3 + \\ \frac{1}{r^4} G^3 \left( -\frac{116}{3} \hat{n} \times \vec{S}_1 \cdot \vec{v}_1 (\hat{n} \cdot \vec{v}_2)^2 + 36 \hat{n} \times \vec{S}_1 \cdot \vec{v}_1 \log \left( \frac{r}{R_0} \right) (\hat{n} \cdot \vec{v}_2)^2 + \frac{944}{75} \vec{S}_1 \times \vec{v}_1 \cdot \vec{v}_2 \hat{n} \cdot \vec{v}_2 + \right. \\ \left. \frac{113}{3} \hat{n} \times \vec{S}_1 \cdot \vec{v}_1 \hat{n} \cdot \vec{v}_1 \hat{n} \cdot \vec{v}_2 - \frac{72}{5} \vec{S}_1 \times \vec{v}_1 \cdot \vec{v}_2 \log \left( \frac{r}{R_0} \right) \hat{n} \cdot \vec{v}_2 - 30 \hat{n} \times \vec{S}_1 \cdot \vec{v}_1 \hat{n} \cdot \vec{v}_1 \log \left( \frac{r}{R_0} \right) \hat{n} \cdot \vec{v}_2 - \right. \\ \left. \frac{19}{3} \vec{S}_1 \times \vec{v}_1 \cdot \vec{v}_2 \hat{n} \cdot \vec{v}_1 - \frac{19}{3} \hat{n} \times \vec{S}_1 \cdot \vec{v}_1 \vec{v}_1 \cdot \vec{v}_2 + \frac{592}{75} \hat{n} \times \vec{S}_1 \cdot \vec{v}_1 \vec{v}_2 \cdot \vec{v}_2 + 6 \vec{S}_1 \times \vec{v}_1 \cdot \vec{v}_2 \hat{n} \cdot \vec{v}_1 \log \left( \frac{r}{R_0} \right) + \right. \\ \left. 6 \hat{n} \times \vec{S}_1 \cdot \vec{v}_1 \vec{v}_1 \cdot \vec{v}_2 \log \left( \frac{r}{R_0} \right) - \frac{36}{5} \hat{n} \times \vec{S}_1 \cdot \vec{v}_1 \vec{v}_2 \cdot \vec{v}_2 \log \left( \frac{r}{R_0} \right) + \frac{1}{\epsilon_d} \left( -12 \hat{n} \times \vec{S}_1 \cdot \vec{v}_1 (\hat{n} \cdot \vec{v}_2)^2 + \frac{24}{5} \vec{S}_1 \times \vec{v}_1 \cdot \vec{v}_2 \hat{n} \cdot \vec{v}_2 + \right. \right. \\ \left. \left. 10 \hat{n} \times \vec{S}_1 \cdot \vec{v}_1 \hat{n} \cdot \vec{v}_1 \hat{n} \cdot \vec{v}_2 - 2 \vec{S}_1 \times \vec{v}_1 \cdot \vec{v}_2 \hat{n} \cdot \vec{v}_1 - 2 \hat{n} \times \vec{S}_1 \cdot \vec{v}_1 \vec{v}_1 \cdot \vec{v}_2 + \frac{12}{5} \hat{n} \times \vec{S}_1 \cdot \vec{v}_1 \vec{v}_2 \cdot \vec{v}_2 \right) \right) m_2^3 \Big\}$$

{DiagSet[3, 1, 124],

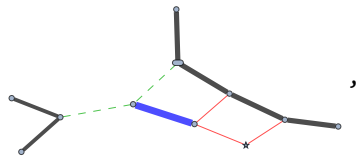

$$\frac{1}{r^3} m_1^2 m_2 \left( \frac{6}{5} \log \left( \frac{r}{R_0} \right) \frac{1}{S_1} \times \vec{v}_1 \cdot \vec{v}_2 - \frac{271}{225} \frac{1}{S_1} \times \vec{v}_1 \cdot \vec{v}_2 - \frac{271}{225} \vec{S}_1 \times \vec{v}_1 \cdot \vec{a}_2 - \frac{143}{75} \hat{n} \times \vec{S}_1 \cdot \vec{v}_1 \hat{n} \cdot \vec{a}_2 - \frac{98}{25} \hat{n} \times \vec{S}_1 \cdot \vec{v}_2 \hat{n} \cdot \vec{v}_1 - \right. \\ \left. \frac{98}{25} \hat{n} \times \vec{S}_1 \cdot \vec{a}_2 \hat{n} \cdot \vec{v}_1 - \frac{143}{75} \hat{n} \times \vec{S}_1 \cdot \vec{v}_1 \hat{n} \cdot \vec{v}_2 + \frac{6}{5} \vec{S}_1 \times \vec{v}_1 \cdot \vec{a}_2 \log \left( \frac{r}{R_0} \right) + \frac{9}{5} \hat{n} \times \vec{S}_1 \cdot \vec{v}_1 \hat{n} \cdot \vec{a}_2 \log \left( \frac{r}{R_0} \right) + \right. \\ \left. \frac{27}{5} \hat{n} \times \vec{S}_1 \cdot \vec{v}_2 \hat{n} \cdot \vec{v}_1 \log \left( \frac{r}{R_0} \right) + \frac{27}{5} \hat{n} \times \vec{S}_1 \cdot \vec{a}_2 \hat{n} \cdot \vec{v}_1 \log \left( \frac{r}{R_0} \right) + \frac{9}{5} \hat{n} \times \vec{S}_1 \cdot \vec{v}_1 \hat{n} \cdot \vec{v}_2 \log \left( \frac{r}{R_0} \right) + \frac{1}{\epsilon_d} \right. \\ \left. \left( -\frac{2}{5} \frac{1}{S_1} \times \vec{v}_1 \cdot \vec{v}_2 - \frac{2}{5} \vec{S}_1 \times \vec{v}_1 \cdot \vec{a}_2 - \frac{3}{5} \hat{n} \times \vec{S}_1 \cdot \vec{v}_1 \hat{n} \cdot \vec{a}_2 - \frac{9}{5} \hat{n} \times \vec{S}_1 \cdot \vec{v}_2 \hat{n} \cdot \vec{v}_1 - \frac{9}{5} \hat{n} \times \vec{S}_1 \cdot \vec{a}_2 \hat{n} \cdot \vec{v}_1 - \frac{3}{5} \hat{n} \times \vec{S}_1 \cdot \vec{v}_1 \hat{n} \cdot \vec{v}_2 \right) \right) \\ G^3 + \frac{1}{r^4} m_1^2 m_2 \left( \frac{3914}{147} \hat{n} \times \vec{S}_1 \cdot \vec{v}_2 (\hat{n} \cdot \vec{v}_1)^2 - \frac{219}{7} \hat{n} \times \vec{S}_1 \cdot \vec{v}_2 \log \left( \frac{r}{R_0} \right) (\hat{n} \cdot \vec{v}_1)^2 + \frac{34619 \vec{S}_1 \times \vec{v}_1 \cdot \vec{v}_2 \hat{n} \cdot \vec{v}_1}{3675} + \right. \\ \left. \frac{496}{49} \hat{n} \times \vec{S}_1 \cdot \vec{v}_1 \hat{n} \cdot \vec{v}_2 \hat{n} \cdot \vec{v}_1 - 25 \hat{n} \times \vec{S}_1 \cdot \vec{v}_2 \hat{n} \cdot \vec{v}_2 \hat{n} \cdot \vec{v}_1 - \frac{381}{35} \vec{S}_1 \times \vec{v}_1 \cdot \vec{v}_2 \log \left( \frac{r}{R_0} \right) \hat{n} \cdot \vec{v}_1 - \right. \\ \left. \frac{57}{7} \hat{n} \times \vec{S}_1 \cdot \vec{v}_1 \hat{n} \cdot \vec{v}_2 \log \left( \frac{r}{R_0} \right) \hat{n} \cdot \vec{v}_1 + 27 \hat{n} \times \vec{S}_1 \cdot \vec{v}_2 \hat{n} \cdot \vec{v}_2 \log \left( \frac{r}{R_0} \right) \hat{n} \cdot \vec{v}_1 - \frac{34}{3} \hat{n} \times \vec{S}_1 \cdot \vec{v}_1 (\hat{n} \cdot \vec{v}_2)^2 - \right. \\ \left. \frac{218}{75} \vec{S}_1 \times \vec{v}_1 \cdot \vec{v}_2 \hat{n} \cdot \vec{v}_2 - \frac{16861 \hat{n} \times \vec{S}_1 \cdot \vec{v}_2 \vec{v}_1 \cdot \vec{v}_1}{3675} - \frac{1661 \hat{n} \times \vec{S}_1 \cdot \vec{v}_1 \vec{v}_1 \cdot \vec{v}_2}{1225} + \frac{98}{25} \hat{n} \times \vec{S}_1 \cdot \vec{v}_2 \vec{v}_1 \cdot \vec{v}_2 + \right. \\ \left. \frac{143}{75} \hat{n} \times \vec{S}_1 \cdot \vec{v}_1 \vec{v}_2 \cdot \vec{v}_2 + 9 \hat{n} \times \vec{S}_1 \cdot \vec{v}_1 (\hat{n} \cdot \vec{v}_2)^2 \log \left( \frac{r}{R_0} \right) + \frac{9}{5} \vec{S}_1 \times \vec{v}_1 \cdot \vec{v}_2 \hat{n} \cdot \vec{v}_2 \log \left( \frac{r}{R_0} \right) + \right. \\ \left. \frac{1}{\epsilon_d} \left( -12 \hat{n} \times \vec{S}_1 \cdot \vec{v}_1 (\hat{n} \cdot \vec{v}_2)^2 + \frac{24}{5} \vec{S}_1 \times \vec{v}_1 \cdot \vec{v}_2 \hat{n} \cdot \vec{v}_2 + 10 \hat{n} \times \vec{S}_1 \cdot \vec{v}_1 \hat{n} \cdot \vec{v}_1 \hat{n} \cdot \vec{v}_2 - 2 \vec{S}_1 \times \vec{v}_1 \cdot \vec{v}_2 \hat{n} \cdot \vec{v}_1 - 2 \hat{n} \times \vec{S}_1 \cdot \vec{v}_1 \vec{v}_1 \cdot \vec{v}_2 + \frac{12}{5} \hat{n} \times \vec{S}_1 \cdot \vec{v}_1 \vec{v}_2 \cdot \vec{v}_2 \right) \right) m_2^3 \Big\}$$

$$\begin{aligned} & \frac{219}{35} \hat{n} \times \vec{S}_1 \cdot \vec{v}_2 \vec{v}_1 \cdot \vec{v}_1 \log\left(\frac{r}{R_0}\right) + \frac{57}{35} \hat{n} \times \vec{S}_1 \cdot \vec{v}_1 \vec{v}_1 \cdot \vec{v}_2 \log\left(\frac{r}{R_0}\right) - \frac{27}{5} \hat{n} \times \vec{S}_1 \cdot \vec{v}_2 \vec{v}_1 \cdot \vec{v}_2 \log\left(\frac{r}{R_0}\right) - \\ & \frac{9}{5} \hat{n} \times \vec{S}_1 \cdot \vec{v}_1 \vec{v}_2 \cdot \vec{v}_2 \log\left(\frac{r}{R_0}\right) + \frac{1}{\epsilon_d} \left( \frac{73}{7} \hat{n} \times \vec{S}_1 \cdot \vec{v}_2 (\hat{n} \cdot \vec{v}_1)^2 + \frac{127}{35} \vec{S}_1 \times \vec{v}_1 \cdot \vec{v}_2 \hat{n} \cdot \vec{v}_1 + \right. \\ & \frac{19}{7} \hat{n} \times \vec{S}_1 \cdot \vec{v}_1 \hat{n} \cdot \vec{v}_2 \hat{n} \cdot \vec{v}_1 - 9 \hat{n} \times \vec{S}_1 \cdot \vec{v}_2 \hat{n} \cdot \vec{v}_2 \hat{n} \cdot \vec{v}_1 - 3 \hat{n} \times \vec{S}_1 \cdot \vec{v}_1 (\hat{n} \cdot \vec{v}_2)^2 - \frac{3}{5} \vec{S}_1 \times \vec{v}_1 \cdot \vec{v}_2 \hat{n} \cdot \vec{v}_2 - \\ & \left. \frac{73}{35} \hat{n} \times \vec{S}_1 \cdot \vec{v}_2 \vec{v}_1 \cdot \vec{v}_1 - \frac{19}{35} \hat{n} \times \vec{S}_1 \cdot \vec{v}_1 \vec{v}_1 \cdot \vec{v}_2 + \frac{9}{5} \hat{n} \times \vec{S}_1 \cdot \vec{v}_2 \vec{v}_1 \cdot \vec{v}_2 + \frac{3}{5} \hat{n} \times \vec{S}_1 \cdot \vec{v}_1 \vec{v}_2 \cdot \vec{v}_2 \right) \Bigg\} G^3 \end{aligned}$$

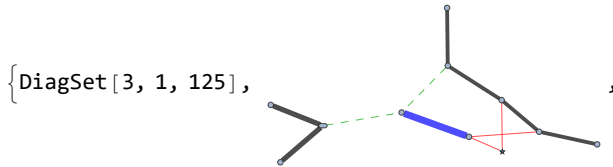

$$\begin{aligned} & \frac{1}{r^3} G^3 m_2^3 \left( \frac{-\frac{2}{5} \hat{n} \cdot \vec{a}_2 \hat{n} \times \vec{S}_1 \cdot \vec{v}_2 - \frac{8}{5} \hat{n} \cdot \vec{v}_2 \hat{n} \times \vec{a}_2 \cdot \vec{S}_1 + \frac{2}{3} \vec{a}_2 \times \vec{S}_1 \cdot \vec{v}_2 + \frac{6}{5} \hat{n} \cdot \vec{v}_2 \hat{n} \times \vec{S}_1 \cdot \vec{v}_2}{\epsilon_d} + \right. \\ & \frac{6}{5} \log\left(\frac{r}{R_0}\right) \hat{n} \cdot \vec{a}_2 \hat{n} \times \vec{S}_1 \cdot \vec{v}_2 + \frac{24}{5} \log\left(\frac{r}{R_0}\right) \hat{n} \cdot \vec{v}_2 \hat{n} \times \vec{a}_2 \cdot \vec{S}_1 - \frac{7}{75} \hat{n} \cdot \vec{a}_2 \hat{n} \times \vec{S}_1 \cdot \vec{v}_2 - \frac{106}{25} \hat{n} \cdot \vec{v}_2 \hat{n} \times \vec{a}_2 \cdot \vec{S}_1 - \\ & \left. 2 \log\left(\frac{r}{R_0}\right) \vec{a}_2 \times \vec{S}_1 \cdot \vec{v}_2 + \frac{7}{9} \vec{a}_2 \times \vec{S}_1 \cdot \vec{v}_2 - \frac{18}{5} \log\left(\frac{r}{R_0}\right) \hat{n} \cdot \vec{v}_2 \hat{n} \times \vec{S}_1 \cdot \vec{v}_2 + \frac{311}{75} \hat{n} \cdot \vec{v}_2 \hat{n} \times \vec{S}_1 \cdot \vec{v}_2 \right) + \frac{1}{r^4} \\ & G^3 m_2^3 \left( \frac{1}{\epsilon_d} \left( \frac{60}{7} (\hat{n} \cdot \vec{v}_2)^2 \hat{n} \times \vec{S}_1 \cdot \vec{v}_2 - \frac{6}{5} \hat{n} \cdot \vec{v}_2 \vec{S}_1 \times \vec{v}_1 \cdot \vec{v}_2 - 6 \hat{n} \cdot \vec{v}_1 \hat{n} \cdot \vec{v}_2 \hat{n} \times \vec{S}_1 \cdot \vec{v}_2 + \frac{6}{5} \vec{v}_1 \cdot \vec{v}_2 \hat{n} \times \vec{S}_1 \cdot \vec{v}_2 - \right. \right. \\ & \frac{12}{7} \vec{v}_2 \cdot \vec{v}_2 \hat{n} \times \vec{S}_1 \cdot \vec{v}_2 \Bigg) - \frac{180}{7} \log\left(\frac{r}{R_0}\right) (\hat{n} \cdot \vec{v}_2)^2 \hat{n} \times \vec{S}_1 \cdot \vec{v}_2 + \frac{18}{5} \log\left(\frac{r}{R_0}\right) \hat{n} \cdot \vec{v}_2 \vec{S}_1 \times \vec{v}_1 \cdot \vec{v}_2 + 18 \log\left(\frac{r}{R_0}\right) \hat{n} \cdot \vec{v}_1 \\ & \hat{n} \cdot \vec{v}_2 \hat{n} \times \vec{S}_1 \cdot \vec{v}_2 - \frac{18}{5} \log\left(\frac{r}{R_0}\right) \vec{v}_1 \cdot \vec{v}_2 \hat{n} \times \vec{S}_1 \cdot \vec{v}_2 + \frac{36}{7} \log\left(\frac{r}{R_0}\right) \vec{v}_2 \cdot \vec{v}_2 \hat{n} \times \vec{S}_1 \cdot \vec{v}_2 + \frac{4192}{147} (\hat{n} \cdot \vec{v}_2)^2 \hat{n} \times \vec{S}_1 \cdot \vec{v}_2 - \\ & \left. \frac{311}{75} \hat{n} \cdot \vec{v}_2 \vec{S}_1 \times \vec{v}_1 \cdot \vec{v}_2 - \frac{73}{3} \hat{n} \cdot \vec{v}_1 \hat{n} \cdot \vec{v}_2 \hat{n} \times \vec{S}_1 \cdot \vec{v}_2 + \frac{311}{75} \vec{v}_1 \cdot \vec{v}_2 \hat{n} \times \vec{S}_1 \cdot \vec{v}_2 - \frac{3352}{735} \vec{v}_2 \cdot \vec{v}_2 \hat{n} \times \vec{S}_1 \cdot \vec{v}_2 \right) \Bigg\} \end{aligned}$$

{DiagSet[3, 1, 126],

,

$$G^3 \left( 2 \log\left(\frac{r}{R_0}\right) \hat{n} \times \vec{S}_1 \cdot \vec{v}_2 - \frac{2 \hat{n} \times \vec{S}_1 \cdot \vec{v}_2}{3 \epsilon_d} - \frac{13}{9} \hat{n} \times \vec{S}_1 \cdot \vec{v}_2 \right) m_2^3 + \frac{1}{r^2}$$

$$\begin{aligned} & \frac{1}{r^3} G^3 \left( -4 \log\left(\frac{r}{R_0}\right) \vec{S}_1 \times \vec{v}_1 \cdot \vec{v}_2 + \frac{26}{9} \vec{S}_1 \times \vec{v}_1 \cdot \vec{v}_2 - \frac{13}{9} \vec{a}_1 \times \vec{S}_1 \cdot \vec{v}_2 + \frac{4}{9} \vec{a}_2 \times \vec{S}_1 \cdot \vec{v}_2 + \frac{19}{3} \hat{n} \times \vec{S}_1 \cdot \vec{v}_2 \hat{n} \cdot \vec{a}_1 - \right. \\ & \frac{361}{150} \hat{n} \times \vec{S}_1 \cdot \vec{v}_2 \hat{n} \cdot \vec{a}_2 + \frac{38}{3} \hat{n} \times \vec{S}_1 \cdot \vec{v}_2 \hat{n} \cdot \vec{v}_1 - \frac{728}{75} \hat{n} \times \vec{S}_1 \cdot \vec{v}_2 \hat{n} \cdot \vec{v}_2 + \frac{161}{150} \hat{n} \times \vec{a}_2 \cdot \vec{S}_1 \hat{n} \cdot \vec{v}_2 + 2 \vec{a}_1 \times \vec{S}_1 \cdot \vec{v}_2 \log\left(\frac{r}{R_0}\right) - \\ & 6 \hat{n} \times \vec{S}_1 \cdot \vec{v}_2 \hat{n} \cdot \vec{a}_1 \log\left(\frac{r}{R_0}\right) + \frac{9}{5} \hat{n} \times \vec{S}_1 \cdot \vec{v}_2 \hat{n} \cdot \vec{a}_2 \log\left(\frac{r}{R_0}\right) - 12 \hat{n} \times \vec{S}_1 \cdot \vec{v}_2 \hat{n} \cdot \vec{v}_1 \log\left(\frac{r}{R_0}\right) + \\ & \frac{54}{5} \hat{n} \times \vec{S}_1 \cdot \vec{v}_2 \hat{n} \cdot \vec{v}_2 \log\left(\frac{r}{R_0}\right) - \frac{9}{5} \hat{n} \times \vec{a}_2 \cdot \vec{S}_1 \hat{n} \cdot \vec{v}_2 \log\left(\frac{r}{R_0}\right) + \frac{1}{\epsilon_d} \left( \frac{4}{3} \vec{S}_1 \times \vec{v}_1 \cdot \vec{v}_2 - \frac{2}{3} \vec{a}_1 \times \vec{S}_1 \cdot \vec{v}_2 + \right. \\ & \left. 2 \hat{n} \times \vec{S}_1 \cdot \vec{v}_2 \hat{n} \cdot \vec{a}_1 - \frac{3}{5} \hat{n} \times \vec{S}_1 \cdot \vec{v}_2 \hat{n} \cdot \vec{a}_2 + 4 \hat{n} \times \vec{S}_1 \cdot \vec{v}_2 \hat{n} \cdot \vec{v}_1 - \frac{18}{5} \hat{n} \times \vec{S}_1 \cdot \vec{v}_2 \hat{n} \cdot \vec{v}_2 + \frac{3}{5} \hat{n} \times \vec{a}_2 \cdot \vec{S}_1 \hat{n} \cdot \vec{v}_2 \right) \Bigg) m_2^3 + \\ & \frac{1}{r^4} G^3 \left( -\frac{113}{3} \hat{n} \times \vec{S}_1 \cdot \vec{v}_2 (\hat{n} \cdot \vec{v}_1)^2 + 30 \hat{n} \times \vec{S}_1 \cdot \vec{v}_2 \log\left(\frac{r}{R_0}\right) (\hat{n} \cdot \vec{v}_1)^2 - \frac{38}{3} \vec{S}_1 \times \vec{v}_1 \cdot \vec{v}_2 \hat{n} \cdot \vec{v}_1 + \right. \end{aligned}$$

$$\begin{aligned} & \frac{178}{3} \hat{n} \times \vec{S}_1 \cdot \vec{v}_2 \hat{n} \cdot \vec{v}_2 \hat{n} \cdot \vec{v}_1 + 12 \vec{S}_1 \times \vec{v}_1 \cdot \vec{v}_2 \log\left(\frac{r}{R_\theta}\right) \hat{n} \cdot \vec{v}_1 - 54 \hat{n} \times \vec{S}_1 \cdot \vec{v}_2 \hat{n} \cdot \vec{v}_2 \log\left(\frac{r}{R_\theta}\right) \hat{n} \cdot \vec{v}_1 - \\ & \frac{3653}{147} \hat{n} \times \vec{S}_1 \cdot \vec{v}_2 (\hat{n} \cdot \vec{v}_2)^2 + \frac{728}{75} \vec{S}_1 \times \vec{v}_1 \cdot \vec{v}_2 \hat{n} \cdot \vec{v}_2 + \frac{19}{3} \hat{n} \times \vec{S}_1 \cdot \vec{v}_2 \vec{v}_1 \cdot \vec{v}_1 - \frac{728}{75} \hat{n} \times \vec{S}_1 \cdot \vec{v}_2 \vec{v}_1 \cdot \vec{v}_2 + \\ & \frac{3107}{735} \hat{n} \times \vec{S}_1 \cdot \vec{v}_2 \vec{v}_2 \cdot \vec{v}_2 + \frac{180}{7} \hat{n} \times \vec{S}_1 \cdot \vec{v}_2 (\hat{n} \cdot \vec{v}_2)^2 \log\left(\frac{r}{R_\theta}\right) - \frac{54}{5} \vec{S}_1 \times \vec{v}_1 \cdot \vec{v}_2 \hat{n} \cdot \vec{v}_2 \log\left(\frac{r}{R_\theta}\right) - \\ & 6 \hat{n} \times \vec{S}_1 \cdot \vec{v}_2 \vec{v}_1 \cdot \vec{v}_1 \log\left(\frac{r}{R_\theta}\right) + \frac{54}{5} \hat{n} \times \vec{S}_1 \cdot \vec{v}_2 \vec{v}_1 \cdot \vec{v}_2 \log\left(\frac{r}{R_\theta}\right) - \frac{36}{7} \hat{n} \times \vec{S}_1 \cdot \vec{v}_2 \vec{v}_2 \cdot \vec{v}_2 \log\left(\frac{r}{R_\theta}\right) + \frac{1}{\epsilon_d} \\ & \left( -10 \hat{n} \times \vec{S}_1 \cdot \vec{v}_2 (\hat{n} \cdot \vec{v}_1)^2 - 4 \vec{S}_1 \times \vec{v}_1 \cdot \vec{v}_2 \hat{n} \cdot \vec{v}_1 + 18 \hat{n} \times \vec{S}_1 \cdot \vec{v}_2 \hat{n} \cdot \vec{v}_2 \hat{n} \cdot \vec{v}_1 - \frac{60}{7} \hat{n} \times \vec{S}_1 \cdot \vec{v}_2 (\hat{n} \cdot \vec{v}_2)^2 + \right. \\ & \left. \frac{18}{5} \vec{S}_1 \times \vec{v}_1 \cdot \vec{v}_2 \hat{n} \cdot \vec{v}_2 + 2 \hat{n} \times \vec{S}_1 \cdot \vec{v}_2 \vec{v}_1 \cdot \vec{v}_1 - \frac{18}{5} \hat{n} \times \vec{S}_1 \cdot \vec{v}_2 \vec{v}_1 \cdot \vec{v}_2 + \frac{12}{7} \hat{n} \times \vec{S}_1 \cdot \vec{v}_2 \vec{v}_2 \cdot \vec{v}_2 \right) m_2^3 \} \end{aligned}$$

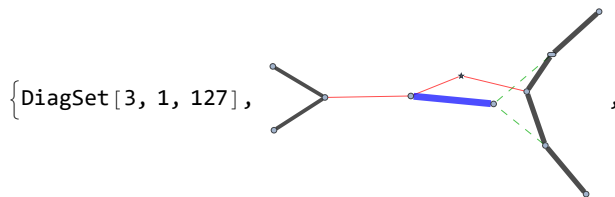

$$\begin{aligned} & \frac{1}{r^3} G^3 m_1^2 m_2 \left( \frac{\frac{3}{5} \hat{n} \cdot \vec{a}_1 \hat{n} \times \vec{S}_1 \cdot \vec{v}_1 + \frac{2}{5} \hat{n} \cdot \vec{v}_1 \hat{n} \times \vec{S}_1 \cdot \vec{a}_1 - \frac{1}{15} \vec{S}_1 \times \vec{v}_1 \cdot \vec{a}_1 + \hat{n} \cdot \vec{v}_1 \hat{n} \times \vec{S}_1 \cdot \vec{v}_1}{\epsilon_d} - \right. \\ & \frac{9}{5} \log\left(\frac{r}{R_\theta}\right) \hat{n} \cdot \vec{a}_1 \hat{n} \times \vec{S}_1 \cdot \vec{v}_1 - \frac{6}{5} \log\left(\frac{r}{R_\theta}\right) \hat{n} \cdot \vec{v}_1 \hat{n} \times \vec{S}_1 \cdot \vec{a}_1 + \frac{31}{25} \hat{n} \cdot \vec{a}_1 \hat{n} \times \vec{S}_1 \cdot \vec{v}_1 + \frac{24}{25} \hat{n} \cdot \vec{v}_1 \hat{n} \times \vec{S}_1 \cdot \vec{a}_1 + \\ & \left. \frac{1}{5} \log\left(\frac{r}{R_\theta}\right) \vec{S}_1 \times \vec{v}_1 \cdot \vec{a}_1 + \frac{1}{25} \vec{S}_1 \times \vec{v}_1 \cdot \vec{a}_1 - 3 \log\left(\frac{r}{R_\theta}\right) \hat{n} \cdot \vec{v}_1 \hat{n} \times \vec{S}_1 \cdot \vec{v}_1 + \frac{11}{5} \hat{n} \cdot \vec{v}_1 \hat{n} \times \vec{S}_1 \cdot \vec{v}_1 \right) + \frac{1}{r^4} G^3 m_1^2 m_2 \\ & \left( \frac{1}{\epsilon_d} \left( -\frac{15}{7} (\hat{n} \cdot \vec{v}_1)^2 \hat{n} \times \vec{S}_1 \cdot \vec{v}_1 - \hat{n} \cdot \vec{v}_1 \vec{S}_1 \times \vec{v}_1 \cdot \vec{v}_2 + 5 \hat{n} \cdot \vec{v}_2 \hat{n} \cdot \vec{v}_1 \hat{n} \times \vec{S}_1 \cdot \vec{v}_1 + \frac{3}{7} \vec{v}_1 \cdot \vec{v}_1 \hat{n} \times \vec{S}_1 \cdot \vec{v}_1 - \vec{v}_1 \cdot \vec{v}_2 \hat{n} \times \vec{S}_1 \cdot \vec{v}_1 \right) + \right. \\ & \frac{45}{7} \log\left(\frac{r}{R_\theta}\right) (\hat{n} \cdot \vec{v}_1)^2 \hat{n} \times \vec{S}_1 \cdot \vec{v}_1 + 3 \log\left(\frac{r}{R_\theta}\right) \hat{n} \cdot \vec{v}_1 \vec{S}_1 \times \vec{v}_1 \cdot \vec{v}_2 - 15 \log\left(\frac{r}{R_\theta}\right) \hat{n} \cdot \vec{v}_2 \hat{n} \cdot \vec{v}_1 \hat{n} \times \vec{S}_1 \cdot \vec{v}_1 - \\ & \frac{9}{7} \log\left(\frac{r}{R_\theta}\right) \vec{v}_1 \cdot \vec{v}_1 \hat{n} \times \vec{S}_1 \cdot \vec{v}_1 + 3 \log\left(\frac{r}{R_\theta}\right) \vec{v}_1 \cdot \vec{v}_2 \hat{n} \times \vec{S}_1 \cdot \vec{v}_1 - \frac{284}{49} (\hat{n} \cdot \vec{v}_1)^2 \hat{n} \times \vec{S}_1 \cdot \vec{v}_1 - \\ & \left. \frac{11}{5} \hat{n} \cdot \vec{v}_1 \vec{S}_1 \times \vec{v}_1 \cdot \vec{v}_2 + 14 \hat{n} \cdot \vec{v}_2 \hat{n} \cdot \vec{v}_1 \hat{n} \times \vec{S}_1 \cdot \vec{v}_1 - \frac{31}{245} \vec{v}_1 \cdot \vec{v}_1 \hat{n} \times \vec{S}_1 \cdot \vec{v}_1 - \frac{11}{5} \vec{v}_1 \cdot \vec{v}_2 \hat{n} \times \vec{S}_1 \cdot \vec{v}_1 \right) \} \end{aligned}$$

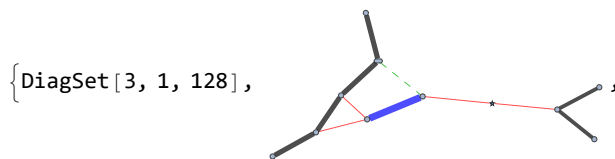

$$\begin{aligned} & \frac{1}{r^3} G^3 m_1^2 m_2 \left( \frac{\frac{3}{10} \hat{n} \cdot \vec{v}_2 \hat{n} \times \vec{S}_1 \cdot \vec{a}_1 - \frac{1}{10} \vec{S}_1 \times \vec{a}_1 \cdot \vec{v}_2 + \frac{3}{10} \hat{n} \cdot \vec{v}_2 \hat{n} \times \vec{S}_1 \cdot \vec{v}_1 - \frac{1}{10} \vec{S}_1 \times \vec{v}_1 \cdot \vec{v}_2}{\epsilon_d} - \right. \\ & \frac{9}{10} \log\left(\frac{r}{R_\theta}\right) \hat{n} \cdot \vec{v}_2 \hat{n} \times \vec{S}_1 \cdot \vec{a}_1 + \frac{41}{50} \hat{n} \cdot \vec{v}_2 \hat{n} \times \vec{S}_1 \cdot \vec{a}_1 + \frac{3}{10} \log\left(\frac{r}{R_\theta}\right) \vec{S}_1 \times \vec{a}_1 \cdot \vec{v}_2 - \frac{13}{75} \vec{S}_1 \times \vec{a}_1 \cdot \vec{v}_2 - \\ & \left. \frac{9}{10} \log\left(\frac{r}{R_\theta}\right) \hat{n} \cdot \vec{v}_2 \hat{n} \times \vec{S}_1 \cdot \vec{v}_1 + \frac{41}{50} \hat{n} \cdot \vec{v}_2 \hat{n} \times \vec{S}_1 \cdot \vec{v}_1 + \frac{3}{10} \log\left(\frac{r}{R_\theta}\right) \vec{S}_1 \times \vec{v}_1 \cdot \vec{v}_2 - \frac{13}{75} \vec{S}_1 \times \vec{v}_1 \cdot \vec{v}_2 \right) + \end{aligned}$$

$$\frac{1}{r^4} G^3 m_1^2 m_2 \left( \frac{\frac{3}{10} \hat{n} \cdot \vec{v}_1 \vec{S}_1 \times \vec{v}_1 \cdot \vec{v}_2 - \frac{3}{2} \hat{n} \cdot \vec{v}_2 \hat{n} \cdot \vec{v}_1 \hat{n} \times \vec{S}_1 \cdot \vec{v}_1 + \frac{3}{10} \vec{v}_1 \cdot \vec{v}_2 \hat{n} \times \vec{S}_1 \cdot \vec{v}_1}{\epsilon_d} - \right. \\ \left. \frac{9}{10} \log\left(\frac{r}{R_\theta}\right) \hat{n} \cdot \vec{v}_1 \vec{S}_1 \times \vec{v}_1 \cdot \vec{v}_2 + \frac{9}{2} \log\left(\frac{r}{R_\theta}\right) \hat{n} \cdot \vec{v}_2 \hat{n} \cdot \vec{v}_1 \hat{n} \times \vec{S}_1 \cdot \vec{v}_1 - \frac{9}{10} \log\left(\frac{r}{R_\theta}\right) \vec{v}_1 \cdot \vec{v}_2 \hat{n} \times \vec{S}_1 \cdot \vec{v}_1 + \right. \\ \left. \frac{41}{50} \hat{n} \cdot \vec{v}_1 \vec{S}_1 \times \vec{v}_1 \cdot \vec{v}_2 - 5 \hat{n} \cdot \vec{v}_2 \hat{n} \cdot \vec{v}_1 \hat{n} \times \vec{S}_1 \cdot \vec{v}_1 + \frac{41}{50} \vec{v}_1 \cdot \vec{v}_2 \hat{n} \times \vec{S}_1 \cdot \vec{v}_1 \right) \Bigg\}$$

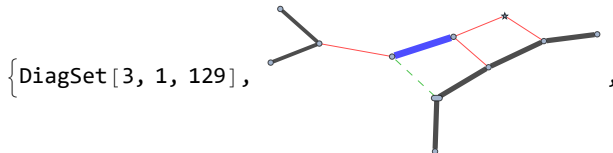

$$\frac{m_1^2 m_2 \left( -\log\left(\frac{r}{R_\theta}\right) \hat{n} \times \vec{S}_1 \cdot \vec{v}_1 + \frac{\hat{n} \times \vec{S}_1 \cdot \vec{v}_1}{3 \epsilon_d} + \frac{11}{18} \hat{n} \times \vec{S}_1 \cdot \vec{v}_1 \right) G^3}{r^2} + \frac{1}{r^3} m_1^2 m_2 \\ \left( 3 \log\left(\frac{r}{R_\theta}\right) \frac{1}{\vec{S}_1 \times \vec{v}_1 \cdot \vec{v}_2} - \frac{14}{9} \frac{1}{\vec{S}_1 \times \vec{v}_1 \cdot \vec{v}_2} + \frac{191}{450} \frac{1}{\vec{S}_1 \times \vec{v}_1 \cdot \vec{v}_1} - \frac{17}{18} \frac{1}{\vec{S}_1 \times \vec{v}_1 \cdot \vec{v}_2} - \frac{34}{15} \hat{n} \times \vec{S}_1 \cdot \vec{v}_1 \hat{n} \cdot \vec{v}_1 + \frac{29}{6} \hat{n} \times \vec{S}_1 \cdot \vec{v}_1 \hat{n} \cdot \vec{v}_2 - \right. \\ \left. \frac{20}{3} \hat{n} \times \vec{S}_1 \cdot \vec{v}_1 \hat{n} \cdot \vec{v}_1 - \frac{119}{150} \hat{n} \times \vec{S}_1 \cdot \vec{v}_1 \hat{n} \cdot \vec{v}_1 + \frac{23}{3} \hat{n} \times \vec{S}_1 \cdot \vec{v}_1 \hat{n} \cdot \vec{v}_2 - \frac{3}{5} \vec{S}_1 \times \vec{v}_1 \cdot \vec{v}_1 \log\left(\frac{r}{R_\theta}\right) + \right. \\ \left. 2 \vec{S}_1 \times \vec{v}_1 \cdot \vec{v}_2 \log\left(\frac{r}{R_\theta}\right) + 3 \hat{n} \times \vec{S}_1 \cdot \vec{v}_1 \hat{n} \cdot \vec{v}_1 \log\left(\frac{r}{R_\theta}\right) - 6 \hat{n} \times \vec{S}_1 \cdot \vec{v}_1 \hat{n} \cdot \vec{v}_2 \log\left(\frac{r}{R_\theta}\right) + 9 \hat{n} \times \vec{S}_1 \cdot \vec{v}_1 \hat{n} \cdot \vec{v}_1 \log\left(\frac{r}{R_\theta}\right) + \right. \\ \left. \frac{6}{5} \hat{n} \times \vec{S}_1 \cdot \vec{v}_1 \hat{n} \cdot \vec{v}_1 \log\left(\frac{r}{R_\theta}\right) - 9 \hat{n} \times \vec{S}_1 \cdot \vec{v}_1 \hat{n} \cdot \vec{v}_2 \log\left(\frac{r}{R_\theta}\right) + \frac{1}{\epsilon_d} \left( -\left(\frac{1}{\vec{S}_1 \times \vec{v}_1 \cdot \vec{v}_2}\right) + \frac{1}{5} \vec{S}_1 \times \vec{v}_1 \cdot \vec{v}_1 - \frac{2}{3} \vec{S}_1 \times \vec{v}_1 \cdot \vec{v}_2 - \right. \right. \\ \left. \left. \hat{n} \times \vec{S}_1 \cdot \vec{v}_1 \hat{n} \cdot \vec{v}_1 + 2 \hat{n} \times \vec{S}_1 \cdot \vec{v}_1 \hat{n} \cdot \vec{v}_2 - 3 \hat{n} \times \vec{S}_1 \cdot \vec{v}_1 \hat{n} \cdot \vec{v}_1 - \frac{2}{5} \hat{n} \times \vec{S}_1 \cdot \vec{v}_1 \hat{n} \cdot \vec{v}_2 + 3 \hat{n} \times \vec{S}_1 \cdot \vec{v}_1 \hat{n} \cdot \vec{v}_2 \right) \right) G^3 + \\ \frac{1}{r^4} m_1^2 m_2 \left( \frac{6319}{294} \hat{n} \times \vec{S}_1 \cdot \vec{v}_1 (\hat{n} \cdot \vec{v}_1)^2 - \frac{180}{7} \hat{n} \times \vec{S}_1 \cdot \vec{v}_1 \log\left(\frac{r}{R_\theta}\right) (\hat{n} \cdot \vec{v}_1)^2 + \frac{578}{75} \vec{S}_1 \times \vec{v}_1 \cdot \vec{v}_2 \hat{n} \cdot \vec{v}_1 - \right. \\ \left. \frac{148}{3} \hat{n} \times \vec{S}_1 \cdot \vec{v}_1 \hat{n} \cdot \vec{v}_2 \hat{n} \cdot \vec{v}_1 - \frac{54}{5} \vec{S}_1 \times \vec{v}_1 \cdot \vec{v}_2 \log\left(\frac{r}{R_\theta}\right) \hat{n} \cdot \vec{v}_1 + 54 \hat{n} \times \vec{S}_1 \cdot \vec{v}_1 \hat{n} \cdot \vec{v}_2 \log\left(\frac{r}{R_\theta}\right) \hat{n} \cdot \vec{v}_1 + \right. \\ \left. \frac{181}{6} \hat{n} \times \vec{S}_1 \cdot \vec{v}_1 (\hat{n} \cdot \vec{v}_2)^2 - \frac{29}{3} \vec{S}_1 \times \vec{v}_1 \cdot \vec{v}_2 \hat{n} \cdot \vec{v}_2 - \frac{5521 \hat{n} \times \vec{S}_1 \cdot \vec{v}_1 \vec{v}_1 \cdot \vec{v}_1}{1470} + \frac{578}{75} \hat{n} \times \vec{S}_1 \cdot \vec{v}_1 \vec{v}_1 \cdot \vec{v}_2 - \right. \\ \left. \frac{29}{6} \hat{n} \times \vec{S}_1 \cdot \vec{v}_1 \vec{v}_2 \cdot \vec{v}_2 - 30 \hat{n} \times \vec{S}_1 \cdot \vec{v}_1 (\hat{n} \cdot \vec{v}_2)^2 \log\left(\frac{r}{R_\theta}\right) + 12 \vec{S}_1 \times \vec{v}_1 \cdot \vec{v}_2 \hat{n} \cdot \vec{v}_2 \log\left(\frac{r}{R_\theta}\right) + \right. \\ \left. \frac{36}{7} \hat{n} \times \vec{S}_1 \cdot \vec{v}_1 \vec{v}_1 \cdot \vec{v}_1 \log\left(\frac{r}{R_\theta}\right) - \frac{54}{5} \hat{n} \times \vec{S}_1 \cdot \vec{v}_1 \vec{v}_1 \cdot \vec{v}_2 \log\left(\frac{r}{R_\theta}\right) + 6 \hat{n} \times \vec{S}_1 \cdot \vec{v}_1 \vec{v}_2 \cdot \vec{v}_2 \log\left(\frac{r}{R_\theta}\right) + \frac{1}{\epsilon_d} \right. \\ \left. \left( \frac{60}{7} \hat{n} \times \vec{S}_1 \cdot \vec{v}_1 (\hat{n} \cdot \vec{v}_1)^2 + \frac{18}{5} \vec{S}_1 \times \vec{v}_1 \cdot \vec{v}_2 \hat{n} \cdot \vec{v}_1 - 18 \hat{n} \times \vec{S}_1 \cdot \vec{v}_1 \hat{n} \cdot \vec{v}_2 \hat{n} \cdot \vec{v}_1 + 10 \hat{n} \times \vec{S}_1 \cdot \vec{v}_1 (\hat{n} \cdot \vec{v}_2)^2 - \right. \right. \\ \left. \left. 4 \vec{S}_1 \times \vec{v}_1 \cdot \vec{v}_2 \hat{n} \cdot \vec{v}_2 - \frac{12}{7} \hat{n} \times \vec{S}_1 \cdot \vec{v}_1 \vec{v}_1 \cdot \vec{v}_1 + \frac{18}{5} \hat{n} \times \vec{S}_1 \cdot \vec{v}_1 \vec{v}_1 \cdot \vec{v}_2 - 2 \hat{n} \times \vec{S}_1 \cdot \vec{v}_1 \vec{v}_2 \cdot \vec{v}_2 \right) \right) G^3 \Bigg\}$$

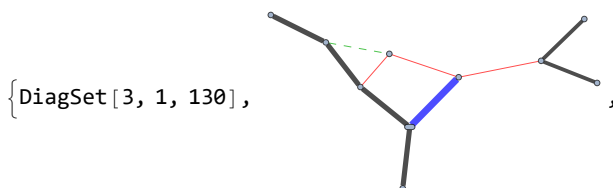



$$\frac{1}{r^3} G^3 m_1^2 m_2 \left( \frac{-\frac{14}{5} \hat{n} \cdot \vec{a}_1 \hat{n} \times \vec{S}_1 \cdot \vec{v}_1 - \frac{4}{5} \hat{n} \cdot \vec{v}_1 \hat{n} \times \vec{S}_1 \cdot \vec{a}_1 + \frac{2}{3} \vec{S}_1 \times \vec{v}_1 \cdot \vec{a}_1 - \frac{18}{5} \hat{n} \cdot \vec{v}_1 \hat{n} \times \vec{S}_1 \cdot \vec{v}_1}{\epsilon_d} + \right.$$

$$\frac{42}{5} \log\left(\frac{r}{R_\theta}\right) \hat{n} \cdot \vec{a}_1 \hat{n} \times \vec{S}_1 \cdot \vec{v}_1 + \frac{12}{5} \log\left(\frac{r}{R_\theta}\right) \hat{n} \cdot \vec{v}_1 \hat{n} \times \vec{S}_1 \cdot \vec{a}_1 - \frac{183}{25} \hat{n} \cdot \vec{a}_1 \hat{n} \times \vec{S}_1 \cdot \vec{v}_1 - \frac{58}{25} \hat{n} \cdot \vec{v}_1 \hat{n} \times \vec{S}_1 \cdot \vec{a}_1 -$$

$$\left. 2 \log\left(\frac{r}{R_\theta}\right) \vec{S}_1 \times \vec{v}_1 \cdot \vec{a}_1 + \vec{S}_1 \times \vec{v}_1 \cdot \vec{a}_1 + \frac{54}{5} \log\left(\frac{r}{R_\theta}\right) \hat{n} \cdot \vec{v}_1 \hat{n} \times \vec{S}_1 \cdot \vec{v}_1 - \frac{241}{25} \hat{n} \cdot \vec{v}_1 \hat{n} \times \vec{S}_1 \cdot \vec{v}_1 \right) +$$

$$\frac{1}{r^4} G^3 m_1^2 m_2 \left( \frac{1}{\epsilon_d} \left( -\frac{82}{7} (\hat{n} \cdot \vec{v}_1)^2 \hat{n} \times \vec{S}_1 \cdot \vec{v}_1 + \frac{18}{5} \hat{n} \cdot \vec{v}_1 \vec{S}_1 \times \vec{v}_1 \cdot \vec{v}_2 - 18 \hat{n} \cdot \vec{v}_2 \hat{n} \cdot \vec{v}_1 \hat{n} \times \vec{S}_1 \cdot \vec{v}_1 + \right.$$

$$\frac{82}{35} \vec{v}_1 \cdot \vec{v}_1 \hat{n} \times \vec{S}_1 \cdot \vec{v}_1 + \frac{18}{5} \vec{v}_1 \cdot \vec{v}_2 \hat{n} \times \vec{S}_1 \cdot \vec{v}_1 \right) + \frac{246}{7} \log\left(\frac{r}{R_\theta}\right) (\hat{n} \cdot \vec{v}_1)^2 \hat{n} \times \vec{S}_1 \cdot \vec{v}_1 -$$

$$\frac{54}{5} \log\left(\frac{r}{R_\theta}\right) \hat{n} \cdot \vec{v}_1 \vec{S}_1 \times \vec{v}_1 \cdot \vec{v}_2 + 54 \log\left(\frac{r}{R_\theta}\right) \hat{n} \cdot \vec{v}_2 \hat{n} \cdot \vec{v}_1 \hat{n} \times \vec{S}_1 \cdot \vec{v}_1 - \frac{246}{35} \log\left(\frac{r}{R_\theta}\right) \vec{v}_1 \cdot \vec{v}_1 \hat{n} \times \vec{S}_1 \cdot \vec{v}_1 -$$

$$\frac{54}{5} \log\left(\frac{r}{R_\theta}\right) \vec{v}_1 \cdot \vec{v}_2 \hat{n} \times \vec{S}_1 \cdot \vec{v}_1 - \frac{2253}{49} (\hat{n} \cdot \vec{v}_1)^2 \hat{n} \times \vec{S}_1 \cdot \vec{v}_1 + \frac{241}{25} \hat{n} \cdot \vec{v}_1 \vec{S}_1 \times \vec{v}_1 \cdot \vec{v}_2 -$$

$$\left. 59 \hat{n} \cdot \vec{v}_2 \hat{n} \cdot \vec{v}_1 \hat{n} \times \vec{S}_1 \cdot \vec{v}_1 + \frac{12063 \vec{v}_1 \cdot \vec{v}_1 \hat{n} \times \vec{S}_1 \cdot \vec{v}_1}{1225} + \frac{241}{25} \vec{v}_1 \cdot \vec{v}_2 \hat{n} \times \vec{S}_1 \cdot \vec{v}_1 \right\}$$

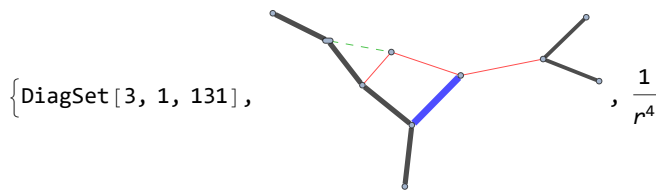

$$G^3 m_1^2 m_2 \left( \frac{4 (\hat{n} \cdot \vec{v}_1)^2 \hat{n} \times \vec{S}_1 \cdot \vec{v}_1 - \frac{4}{5} \vec{v}_1 \cdot \vec{v}_1 \hat{n} \times \vec{S}_1 \cdot \vec{v}_1}{\epsilon_d} - 12 \log\left(\frac{r}{R_\theta}\right) (\hat{n} \cdot \vec{v}_1)^2 \hat{n} \times \vec{S}_1 \cdot \vec{v}_1 + \right.$$

$$\left. \frac{12}{5} \log\left(\frac{r}{R_\theta}\right) \vec{v}_1 \cdot \vec{v}_1 \hat{n} \times \vec{S}_1 \cdot \vec{v}_1 + 6 (\hat{n} \cdot \vec{v}_1)^2 \hat{n} \times \vec{S}_1 \cdot \vec{v}_1 - \frac{18}{25} \vec{v}_1 \cdot \vec{v}_1 \hat{n} \times \vec{S}_1 \cdot \vec{v}_1 \right\}$$

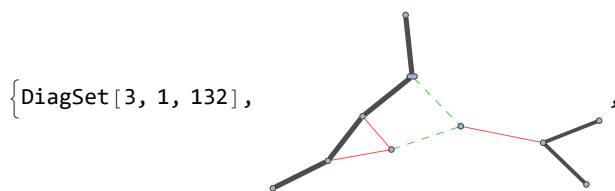

$$\frac{1}{r^3} G^3 m_1^2 m_2 \left( \frac{\frac{2}{5} \hat{n} \cdot \vec{v}_1 \hat{n} \times \vec{S}_1 \cdot \vec{a}_1 + \frac{2}{15} \vec{S}_1 \times \vec{v}_1 \cdot \vec{a}_1 + \frac{2}{5} \hat{n} \cdot \vec{v}_1 \hat{n} \times \vec{S}_1 \cdot \vec{v}_1}{\epsilon_d} - \frac{6}{5} \log\left(\frac{r}{R_\theta}\right) \hat{n} \cdot \vec{v}_1 \hat{n} \times \vec{S}_1 \cdot \vec{a}_1 + \frac{24}{25} \hat{n} \cdot \vec{v}_1 \hat{n} \times \vec{S}_1 \cdot \vec{a}_1 - \right.$$

$$\left. \frac{2}{5} \log\left(\frac{r}{R_\theta}\right) \vec{S}_1 \times \vec{v}_1 \cdot \vec{a}_1 - \frac{46}{75} \vec{S}_1 \times \vec{v}_1 \cdot \vec{a}_1 - \frac{6}{5} \log\left(\frac{r}{R_\theta}\right) \hat{n} \cdot \vec{v}_1 \hat{n} \times \vec{S}_1 \cdot \vec{v}_1 + \frac{24}{25} \hat{n} \cdot \vec{v}_1 \hat{n} \times \vec{S}_1 \cdot \vec{v}_1 \right) +$$

$$\frac{1}{r^4} G^3 m_1^2 m_2 \left( \frac{\frac{6}{35} \vec{v}_1 \cdot \vec{v}_1 \hat{n} \times \vec{S}_1 \cdot \vec{v}_1 - \frac{6}{7} (\hat{n} \cdot \vec{v}_1)^2 \hat{n} \times \vec{S}_1 \cdot \vec{v}_1}{\epsilon_d} + \frac{18}{7} \log\left(\frac{r}{R_\theta}\right) (\hat{n} \cdot \vec{v}_1)^2 \hat{n} \times \vec{S}_1 \cdot \vec{v}_1 - \right.$$

$$\frac{18}{35} \log\left(\frac{r}{R_\theta}\right) \vec{v}_1 \cdot \vec{v}_1 \hat{n} \times \vec{S}_1 \cdot \vec{v}_1 - \frac{122}{49} (\hat{n} \cdot \vec{v}_1)^2 \hat{n} \times \vec{S}_1 \cdot \vec{v}_1 - \frac{2637 \vec{v}_1 \cdot \vec{v}_1 \hat{n} \times \vec{S}_1 \cdot \vec{v}_1}{2450} - \frac{3}{10} \vec{v}_2 \cdot \vec{v}_2 \hat{n} \times \vec{S}_1 \cdot \vec{v}_1 \Bigg\}$$

$$\left\{ \text{DiagSet}[3, 1, 133], \frac{1}{r^4} \right\}$$

$$G^3 m_1^2 m_2 \left( \frac{-\frac{4}{5} \hat{n} \cdot \vec{v}_1 \vec{S}_1 \times \vec{v}_1 \cdot \vec{v}_2 + 4 \hat{n} \cdot \vec{v}_2 \hat{n} \cdot \vec{v}_1 \hat{n} \times \vec{S}_1 \cdot \vec{v}_1 - \frac{4}{5} \vec{v}_1 \cdot \vec{v}_2 \hat{n} \times \vec{S}_1 \cdot \vec{v}_1}{\epsilon_d} + \right. \\ \left. \frac{12}{5} \log\left(\frac{r}{R_\theta}\right) \hat{n} \cdot \vec{v}_1 \vec{S}_1 \times \vec{v}_1 \cdot \vec{v}_2 - 12 \log\left(\frac{r}{R_\theta}\right) \hat{n} \cdot \vec{v}_2 \hat{n} \cdot \vec{v}_1 \hat{n} \times \vec{S}_1 \cdot \vec{v}_1 + \frac{12}{5} \log\left(\frac{r}{R_\theta}\right) \vec{v}_1 \cdot \vec{v}_2 \hat{n} \times \vec{S}_1 \cdot \vec{v}_1 - \right. \\ \left. \frac{58}{25} \hat{n} \cdot \vec{v}_1 \vec{S}_1 \times \vec{v}_1 \cdot \vec{v}_2 + 10 \hat{n} \cdot \vec{v}_2 \hat{n} \cdot \vec{v}_1 \hat{n} \times \vec{S}_1 \cdot \vec{v}_1 + \frac{22}{25} \vec{v}_1 \cdot \vec{v}_2 \hat{n} \times \vec{S}_1 \cdot \vec{v}_1 \right\}$$

$$\left\{ \text{DiagSet}[3, 1, 134], \frac{1}{r^4} G^3 m_1^2 m_2 \right\}$$

$$\left( \frac{1}{\epsilon_d} \left( -4 (\hat{n} \cdot \vec{v}_1)^2 \hat{n} \times \vec{S}_1 \cdot \vec{v}_1 + \frac{4}{5} \hat{n} \cdot \vec{v}_1 \vec{S}_1 \times \vec{v}_1 \cdot \vec{v}_2 - 4 \hat{n} \cdot \vec{v}_2 \hat{n} \cdot \vec{v}_1 \hat{n} \times \vec{S}_1 \cdot \vec{v}_1 + \frac{4}{5} \vec{v}_1 \cdot \vec{v}_1 \hat{n} \times \vec{S}_1 \cdot \vec{v}_1 + \frac{4}{5} \vec{v}_1 \cdot \vec{v}_2 \hat{n} \times \vec{S}_1 \cdot \vec{v}_1 \right) + \right. \\ \left. 12 \log\left(\frac{r}{R_\theta}\right) (\hat{n} \cdot \vec{v}_1)^2 \hat{n} \times \vec{S}_1 \cdot \vec{v}_1 - \frac{12}{5} \log\left(\frac{r}{R_\theta}\right) \hat{n} \cdot \vec{v}_1 \vec{S}_1 \times \vec{v}_1 \cdot \vec{v}_2 + 12 \log\left(\frac{r}{R_\theta}\right) \hat{n} \cdot \vec{v}_2 \hat{n} \cdot \vec{v}_1 \hat{n} \times \vec{S}_1 \cdot \vec{v}_1 - \right. \\ \left. \frac{12}{5} \log\left(\frac{r}{R_\theta}\right) \vec{v}_1 \cdot \vec{v}_1 \hat{n} \times \vec{S}_1 \cdot \vec{v}_1 - \frac{12}{5} \log\left(\frac{r}{R_\theta}\right) \vec{v}_1 \cdot \vec{v}_2 \hat{n} \times \vec{S}_1 \cdot \vec{v}_1 - 10 (\hat{n} \cdot \vec{v}_1)^2 \hat{n} \times \vec{S}_1 \cdot \vec{v}_1 + \right. \\ \left. \frac{38}{25} \hat{n} \cdot \vec{v}_1 \vec{S}_1 \times \vec{v}_1 \cdot \vec{v}_2 - 10 \hat{n} \cdot \vec{v}_2 \hat{n} \cdot \vec{v}_1 \hat{n} \times \vec{S}_1 \cdot \vec{v}_1 + \frac{58}{25} \vec{v}_1 \cdot \vec{v}_1 \hat{n} \times \vec{S}_1 \cdot \vec{v}_1 + \frac{38}{25} \vec{v}_1 \cdot \vec{v}_2 \hat{n} \times \vec{S}_1 \cdot \vec{v}_1 \right) \Bigg\}$$

$$\left\{ \text{DiagSet}[3, 1, 135], \frac{1}{r^4} \right\}$$

$$G^3 m_2^3 \left( \frac{-4 (\hat{n} \cdot \vec{v}_2)^2 \hat{n} \times \vec{S}_1 \cdot \vec{v}_1 + \frac{8}{5} \hat{n} \cdot \vec{v}_2 \vec{S}_1 \times \vec{v}_1 \cdot \vec{v}_2 + \frac{4}{5} \vec{v}_2 \cdot \vec{v}_2 \hat{n} \times \vec{S}_1 \cdot \vec{v}_1}{\epsilon_d} + \right. \\ \left. 12 \log\left(\frac{r}{R_\theta}\right) (\hat{n} \cdot \vec{v}_2)^2 \hat{n} \times \vec{S}_1 \cdot \vec{v}_1 - \frac{24}{5} \log\left(\frac{r}{R_\theta}\right) \hat{n} \cdot \vec{v}_2 \vec{S}_1 \times \vec{v}_1 \cdot \vec{v}_2 - \frac{12}{5} \log\left(\frac{r}{R_\theta}\right) \vec{v}_2 \cdot \vec{v}_2 \hat{n} \times \vec{S}_1 \cdot \vec{v}_1 - \right. \\ \left. 10 (\hat{n} \cdot \vec{v}_2)^2 \hat{n} \times \vec{S}_1 \cdot \vec{v}_1 + \frac{76}{25} \hat{n} \cdot \vec{v}_2 \vec{S}_1 \times \vec{v}_1 \cdot \vec{v}_2 - \frac{82}{25} \vec{v}_2 \cdot \vec{v}_2 \hat{n} \times \vec{S}_1 \cdot \vec{v}_1 \right) \Bigg\}$$

{DiagSet[3, 1, 136],

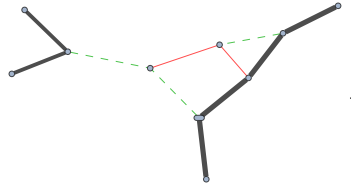

,

$$\begin{aligned} & \frac{1}{r^3} m_1^2 m_2 \left( -\frac{32}{5} \log\left(\frac{r}{R_\theta}\right) \vec{S}_1 \times \vec{v}_1 \cdot \vec{v}_2 + \frac{224}{75} \vec{S}_1 \times \vec{v}_1 \cdot \vec{v}_2 + \frac{224}{75} \vec{S}_1 \times \vec{v}_1 \cdot \vec{a}_2 - \frac{208}{25} \hat{n} \times \vec{S}_1 \cdot \vec{v}_1 \hat{n} \cdot \vec{a}_2 - \frac{64}{25} \hat{n} \times \vec{S}_1 \cdot \vec{v}_2 \hat{n} \cdot \vec{v}_1 - \right. \\ & \frac{64}{25} \hat{n} \times \vec{S}_1 \cdot \vec{a}_2 \hat{n} \cdot \vec{v}_1 - \frac{208}{25} \hat{n} \times \vec{S}_1 \cdot \vec{v}_1 \hat{n} \cdot \vec{v}_2 - \frac{32}{5} \vec{S}_1 \times \vec{v}_1 \cdot \vec{a}_2 \log\left(\frac{r}{R_\theta}\right) + \frac{72}{5} \hat{n} \times \vec{S}_1 \cdot \vec{v}_1 \hat{n} \cdot \vec{a}_2 \log\left(\frac{r}{R_\theta}\right) - \\ & \frac{24}{5} \hat{n} \times \vec{S}_1 \cdot \vec{v}_2 \hat{n} \cdot \vec{v}_1 \log\left(\frac{r}{R_\theta}\right) - \frac{24}{5} \hat{n} \times \vec{S}_1 \cdot \vec{a}_2 \hat{n} \cdot \vec{v}_1 \log\left(\frac{r}{R_\theta}\right) + \frac{72}{5} \hat{n} \times \vec{S}_1 \cdot \vec{v}_1 \hat{n} \cdot \vec{v}_2 \log\left(\frac{r}{R_\theta}\right) + \frac{1}{\epsilon_d} \left( \frac{32}{15} \vec{S}_1 \times \vec{v}_1 \cdot \vec{v}_2 + \right. \\ & \frac{32}{15} \vec{S}_1 \times \vec{v}_1 \cdot \vec{a}_2 - \frac{24}{5} \hat{n} \times \vec{S}_1 \cdot \vec{v}_1 \hat{n} \cdot \vec{a}_2 + \frac{8}{5} \hat{n} \times \vec{S}_1 \cdot \vec{v}_2 \hat{n} \cdot \vec{v}_1 + \frac{8}{5} \hat{n} \times \vec{S}_1 \cdot \vec{a}_2 \hat{n} \cdot \vec{v}_1 - \frac{24}{5} \hat{n} \times \vec{S}_1 \cdot \vec{v}_1 \hat{n} \cdot \vec{v}_2 \left. \right) \Big) G^3 + \\ & \frac{1}{r^4} m_1^2 m_2 \left( \frac{648}{49} \hat{n} \times \vec{S}_1 \cdot \vec{v}_2 (\hat{n} \cdot \vec{v}_1)^2 - \frac{24}{7} \hat{n} \times \vec{S}_1 \cdot \vec{v}_2 \log\left(\frac{r}{R_\theta}\right) (\hat{n} \cdot \vec{v}_1)^2 + \frac{3968}{245} \vec{S}_1 \times \vec{v}_1 \cdot \vec{v}_2 \hat{n} \cdot \vec{v}_1 - \right. \\ & \frac{1160}{49} \hat{n} \times \vec{S}_1 \cdot \vec{v}_1 \hat{n} \cdot \vec{v}_2 \hat{n} \cdot \vec{v}_1 - 8 \hat{n} \times \vec{S}_1 \cdot \vec{v}_2 \hat{n} \cdot \vec{v}_2 \hat{n} \cdot \vec{v}_1 - \frac{24}{7} \vec{S}_1 \times \vec{v}_1 \cdot \vec{v}_2 \log\left(\frac{r}{R_\theta}\right) \hat{n} \cdot \vec{v}_1 + \\ & \frac{72}{7} \hat{n} \times \vec{S}_1 \cdot \vec{v}_1 \hat{n} \cdot \vec{v}_2 \log\left(\frac{r}{R_\theta}\right) \hat{n} \cdot \vec{v}_1 - 24 \hat{n} \times \vec{S}_1 \cdot \vec{v}_2 \hat{n} \cdot \vec{v}_2 \log\left(\frac{r}{R_\theta}\right) \hat{n} \cdot \vec{v}_1 - 56 \hat{n} \times \vec{S}_1 \cdot \vec{v}_1 (\hat{n} \cdot \vec{v}_2)^2 + \\ & \frac{592}{25} \vec{S}_1 \times \vec{v}_1 \cdot \vec{v}_2 \hat{n} \cdot \vec{v}_2 + \frac{7008 \hat{n} \times \vec{S}_1 \cdot \vec{v}_2 \vec{v}_1 \cdot \vec{v}_1}{1225} - \frac{1424 \hat{n} \times \vec{S}_1 \cdot \vec{v}_1 \vec{v}_1 \cdot \vec{v}_2}{1225} + \frac{64}{25} \hat{n} \times \vec{S}_1 \cdot \vec{v}_2 \vec{v}_1 \cdot \vec{v}_2 + \\ & \frac{208}{25} \hat{n} \times \vec{S}_1 \cdot \vec{v}_1 \vec{v}_2 \cdot \vec{v}_2 + 72 \hat{n} \times \vec{S}_1 \cdot \vec{v}_1 (\hat{n} \cdot \vec{v}_2)^2 \log\left(\frac{r}{R_\theta}\right) - \frac{168}{5} \vec{S}_1 \times \vec{v}_1 \cdot \vec{v}_2 \hat{n} \cdot \vec{v}_2 \log\left(\frac{r}{R_\theta}\right) + \\ & \frac{24}{35} \hat{n} \times \vec{S}_1 \cdot \vec{v}_2 \vec{v}_1 \cdot \vec{v}_1 \log\left(\frac{r}{R_\theta}\right) - \frac{72}{35} \hat{n} \times \vec{S}_1 \cdot \vec{v}_1 \vec{v}_1 \cdot \vec{v}_2 \log\left(\frac{r}{R_\theta}\right) + \frac{24}{5} \hat{n} \times \vec{S}_1 \cdot \vec{v}_2 \vec{v}_1 \cdot \vec{v}_2 \log\left(\frac{r}{R_\theta}\right) - \\ & \frac{72}{5} \hat{n} \times \vec{S}_1 \cdot \vec{v}_1 \vec{v}_2 \cdot \vec{v}_2 \log\left(\frac{r}{R_\theta}\right) + \frac{1}{\epsilon_d} \left( \frac{8}{7} \hat{n} \times \vec{S}_1 \cdot \vec{v}_2 (\hat{n} \cdot \vec{v}_1)^2 + \frac{8}{7} \vec{S}_1 \times \vec{v}_1 \cdot \vec{v}_2 \hat{n} \cdot \vec{v}_1 - \right. \\ & \frac{24}{7} \hat{n} \times \vec{S}_1 \cdot \vec{v}_1 \hat{n} \cdot \vec{v}_2 \hat{n} \cdot \vec{v}_1 + 8 \hat{n} \times \vec{S}_1 \cdot \vec{v}_2 \hat{n} \cdot \vec{v}_2 \hat{n} \cdot \vec{v}_1 - 24 \hat{n} \times \vec{S}_1 \cdot \vec{v}_1 (\hat{n} \cdot \vec{v}_2)^2 + \frac{56}{5} \vec{S}_1 \times \vec{v}_1 \cdot \vec{v}_2 \hat{n} \cdot \vec{v}_2 - \\ & \left. \frac{8}{35} \hat{n} \times \vec{S}_1 \cdot \vec{v}_2 \vec{v}_1 \cdot \vec{v}_1 + \frac{24}{35} \hat{n} \times \vec{S}_1 \cdot \vec{v}_1 \vec{v}_1 \cdot \vec{v}_2 - \frac{8}{5} \hat{n} \times \vec{S}_1 \cdot \vec{v}_2 \vec{v}_1 \cdot \vec{v}_2 + \frac{24}{5} \hat{n} \times \vec{S}_1 \cdot \vec{v}_1 \vec{v}_2 \cdot \vec{v}_2 \right) \Big) G^3 \Big\} \end{aligned}$$

{DiagSet[3, 1, 137],

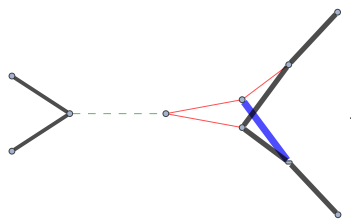

,

$$\begin{aligned} & \frac{1}{r^3} G^3 m_1^2 m_2 \left( \frac{\frac{1}{5} \hat{n} \cdot \vec{v}_2 \hat{n} \times \vec{S}_1 \cdot \vec{a}_1 - \frac{1}{15} \vec{S}_1 \times \vec{a}_1 \cdot \vec{v}_2 + \frac{1}{5} \hat{n} \cdot \vec{v}_2 \hat{n} \times \vec{S}_1 \cdot \vec{v}_1 - \frac{1}{15} \vec{S}_1 \times \vec{v}_1 \cdot \vec{v}_2}{\epsilon_d} - \right. \\ & \frac{3}{5} \log\left(\frac{r}{R_\theta}\right) \hat{n} \cdot \vec{v}_2 \hat{n} \times \vec{S}_1 \cdot \vec{a}_1 + \frac{7}{25} \hat{n} \cdot \vec{v}_2 \hat{n} \times \vec{S}_1 \cdot \vec{a}_1 + \frac{1}{5} \log\left(\frac{r}{R_\theta}\right) \vec{S}_1 \times \vec{a}_1 \cdot \vec{v}_2 + \frac{1}{25} \vec{S}_1 \times \vec{a}_1 \cdot \vec{v}_2 - \\ & \left. \frac{3}{5} \log\left(\frac{r}{R_\theta}\right) \hat{n} \cdot \vec{v}_2 \hat{n} \times \vec{S}_1 \cdot \vec{v}_1 + \frac{7}{25} \hat{n} \cdot \vec{v}_2 \hat{n} \times \vec{S}_1 \cdot \vec{v}_1 + \frac{1}{5} \log\left(\frac{r}{R_\theta}\right) \vec{S}_1 \times \vec{v}_1 \cdot \vec{v}_2 + \frac{1}{25} \vec{S}_1 \times \vec{v}_1 \cdot \vec{v}_2 \right) + \end{aligned}$$

$$\frac{1}{r^4} G^3 m_1^2 m_2 \left( \frac{\frac{8}{35} \hat{n} \cdot \vec{v}_1 \vec{S}_1 \times \vec{v}_1 \cdot \vec{v}_2 - \frac{8}{7} \hat{n} \cdot \vec{v}_2 \hat{n} \cdot \vec{v}_1 \hat{n} \times \vec{S}_1 \cdot \vec{v}_1 + \frac{8}{35} \vec{v}_1 \cdot \vec{v}_2 \hat{n} \times \vec{S}_1 \cdot \vec{v}_1}{\epsilon_d} - \frac{24}{35} \log\left(\frac{r}{R_\theta}\right) \hat{n} \cdot \vec{v}_1 \vec{S}_1 \times \vec{v}_1 \cdot \vec{v}_2 + \frac{24}{7} \log\left(\frac{r}{R_\theta}\right) \hat{n} \cdot \vec{v}_2 \hat{n} \cdot \vec{v}_1 \hat{n} \times \vec{S}_1 \cdot \vec{v}_1 - \frac{24}{35} \log\left(\frac{r}{R_\theta}\right) \vec{v}_1 \cdot \vec{v}_2 \hat{n} \times \vec{S}_1 \cdot \vec{v}_1 + \frac{377 \hat{n} \cdot \vec{v}_1 \vec{S}_1 \times \vec{v}_1 \cdot \vec{v}_2}{1225} - \frac{116}{49} \hat{n} \cdot \vec{v}_2 \hat{n} \cdot \vec{v}_1 \hat{n} \times \vec{S}_1 \cdot \vec{v}_1 + \frac{132 \vec{v}_1 \cdot \vec{v}_2 \hat{n} \times \vec{S}_1 \cdot \vec{v}_1}{1225} \right) \Bigg\}$$

{DiagSet[3, 1, 138],

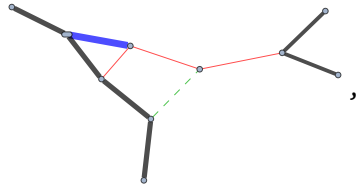

$$\frac{1}{r^3} G^3 m_1^2 m_2 \left( \frac{-\hat{n} \cdot \vec{v}_1 \hat{n} \times \vec{S}_1 \cdot \vec{a}_1 - \frac{1}{3} \vec{S}_1 \times \vec{v}_1 \cdot \vec{a}_1 - \hat{n} \cdot \vec{v}_1 \hat{n} \times \vec{S}_1 \cdot \vec{v}_1}{\epsilon_d} + 3 \log\left(\frac{r}{R_\theta}\right) \hat{n} \cdot \vec{v}_1 \hat{n} \times \vec{S}_1 \cdot \vec{a}_1 - \hat{n} \cdot \vec{v}_1 \hat{n} \times \vec{S}_1 \cdot \vec{a}_1 + \right.$$

$$\left. \log\left(\frac{r}{R_\theta}\right) \vec{S}_1 \times \vec{v}_1 \cdot \vec{a}_1 + 3 \log\left(\frac{r}{R_\theta}\right) \hat{n} \cdot \vec{v}_1 \hat{n} \times \vec{S}_1 \cdot \vec{v}_1 + \hat{n} \cdot \vec{v}_1 \left( -\left( \hat{n} \times \vec{S}_1 \cdot \vec{v}_1 \right) \right) \right) + \frac{1}{r^4} G^3 m_1^2 m_2$$

$$\left( \frac{1}{\epsilon_d} \left( 4 (\hat{n} \cdot \vec{v}_1)^2 \hat{n} \times \vec{S}_1 \cdot \vec{v}_1 - \frac{4}{5} \hat{n} \cdot \vec{v}_1 \vec{S}_1 \times \vec{v}_1 \cdot \vec{v}_2 + 4 \hat{n} \cdot \vec{v}_2 \hat{n} \cdot \vec{v}_1 \hat{n} \times \vec{S}_1 \cdot \vec{v}_1 - \frac{4}{5} \vec{v}_1 \cdot \vec{v}_1 \hat{n} \times \vec{S}_1 \cdot \vec{v}_1 - \frac{4}{5} \vec{v}_1 \cdot \vec{v}_2 \hat{n} \times \vec{S}_1 \cdot \vec{v}_1 \right) - 12 \log\left(\frac{r}{R_\theta}\right) (\hat{n} \cdot \vec{v}_1)^2 \hat{n} \times \vec{S}_1 \cdot \vec{v}_1 + \frac{12}{5} \log\left(\frac{r}{R_\theta}\right) \hat{n} \cdot \vec{v}_1 \vec{S}_1 \times \vec{v}_1 \cdot \vec{v}_2 - 12 \log\left(\frac{r}{R_\theta}\right) \hat{n} \cdot \vec{v}_2 \hat{n} \cdot \vec{v}_1 \hat{n} \times \vec{S}_1 \cdot \vec{v}_1 + \frac{12}{5} \log\left(\frac{r}{R_\theta}\right) \vec{v}_1 \cdot \vec{v}_1 \hat{n} \times \vec{S}_1 \cdot \vec{v}_1 + \frac{12}{5} \log\left(\frac{r}{R_\theta}\right) \vec{v}_1 \cdot \vec{v}_2 \hat{n} \times \vec{S}_1 \cdot \vec{v}_1 + 6 (\hat{n} \cdot \vec{v}_1)^2 \hat{n} \times \vec{S}_1 \cdot \vec{v}_1 - \frac{18}{25} \hat{n} \cdot \vec{v}_1 \vec{S}_1 \times \vec{v}_1 \cdot \vec{v}_2 + 6 \hat{n} \cdot \vec{v}_2 \hat{n} \cdot \vec{v}_1 \hat{n} \times \vec{S}_1 \cdot \vec{v}_1 - \frac{18}{25} \vec{v}_1 \cdot \vec{v}_1 \hat{n} \times \vec{S}_1 \cdot \vec{v}_1 - \frac{18}{25} \vec{v}_1 \cdot \vec{v}_2 \hat{n} \times \vec{S}_1 \cdot \vec{v}_1 \right) \Bigg\}$$

{DiagSet[3, 1, 139],

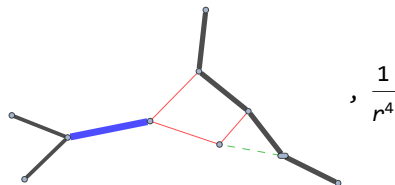

,  $\frac{1}{r^4}$

$$G^3 m_1^2 m_2 \left( \frac{-\frac{4}{7} (\hat{n} \cdot \vec{v}_2)^2 \hat{n} \times \vec{S}_1 \cdot \vec{v}_1 + \frac{8}{35} \hat{n} \cdot \vec{v}_2 \vec{S}_1 \times \vec{v}_1 \cdot \vec{v}_2 + \frac{4}{35} \vec{v}_2 \cdot \vec{v}_2 \hat{n} \times \vec{S}_1 \cdot \vec{v}_1}{\epsilon_d} + \frac{12}{7} \log\left(\frac{r}{R_\theta}\right) (\hat{n} \cdot \vec{v}_2)^2 \hat{n} \times \vec{S}_1 \cdot \vec{v}_1 - \frac{24}{35} \log\left(\frac{r}{R_\theta}\right) \hat{n} \cdot \vec{v}_2 \vec{S}_1 \times \vec{v}_1 \cdot \vec{v}_2 - \frac{12}{35} \log\left(\frac{r}{R_\theta}\right) \vec{v}_2 \cdot \vec{v}_2 \hat{n} \times \vec{S}_1 \cdot \vec{v}_1 - \frac{58}{49} (\hat{n} \cdot \vec{v}_2)^2 \hat{n} \times \vec{S}_1 \cdot \vec{v}_1 + \frac{377 \hat{n} \cdot \vec{v}_2 \vec{S}_1 \times \vec{v}_1 \cdot \vec{v}_2}{1225} + \frac{66 \vec{v}_2 \cdot \vec{v}_2 \hat{n} \times \vec{S}_1 \cdot \vec{v}_1}{1225} \right) \Bigg\}$$

{DiagSet[3, 1, 140],

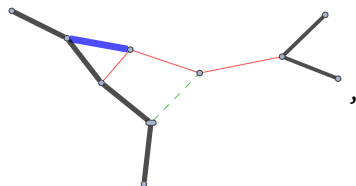

$$\frac{1}{r^3} G^3 m_1^2 m_2 \left( \frac{\frac{8}{5} \hat{n} \cdot \vec{a}_1 \hat{n} \times \vec{S}_1 \cdot \vec{v}_1 + \frac{8}{5} \hat{n} \cdot \vec{v}_1 \hat{n} \times \vec{S}_1 \cdot \vec{a}_1}{\epsilon_d} - \frac{24}{5} \log\left(\frac{r}{R_\theta}\right) \hat{n} \cdot \vec{a}_1 \hat{n} \times \vec{S}_1 \cdot \vec{v}_1 - \right.$$

$$\left. \frac{24}{5} \log\left(\frac{r}{R_\theta}\right) \hat{n} \cdot \vec{v}_1 \hat{n} \times \vec{S}_1 \cdot \vec{a}_1 + \frac{116}{25} \hat{n} \cdot \vec{a}_1 \hat{n} \times \vec{S}_1 \cdot \vec{v}_1 + \frac{116}{25} \hat{n} \cdot \vec{v}_1 \hat{n} \times \vec{S}_1 \cdot \vec{a}_1 \right) + \frac{1}{r^4}$$

$$G^3 m_1^2 m_2 \left( \frac{1}{\epsilon_d} \left( -\frac{48}{7} (\hat{n} \cdot \vec{v}_1)^2 \hat{n} \times \vec{S}_1 \cdot \vec{v}_1 + \frac{8}{5} \hat{n} \cdot \vec{v}_1 \vec{S}_1 \times \vec{v}_1 \cdot \vec{v}_2 - 8 \hat{n} \cdot \vec{v}_2 \hat{n} \cdot \vec{v}_1 \hat{n} \times \vec{S}_1 \cdot \vec{v}_1 + \frac{48}{35} \vec{v}_1 \cdot \vec{v}_1 \hat{n} \times \vec{S}_1 \cdot \vec{v}_1 + \right. \right.$$

$$\left. \frac{8}{5} \vec{v}_1 \cdot \vec{v}_2 \hat{n} \times \vec{S}_1 \cdot \vec{v}_1 \right) + \frac{144}{7} \log\left(\frac{r}{R_\theta}\right) (\hat{n} \cdot \vec{v}_1)^2 \hat{n} \times \vec{S}_1 \cdot \vec{v}_1 - \frac{24}{5} \log\left(\frac{r}{R_\theta}\right) \hat{n} \cdot \vec{v}_1 \vec{S}_1 \times \vec{v}_1 \cdot \vec{v}_2 + 24 \log\left(\frac{r}{R_\theta}\right) \hat{n} \cdot \vec{v}_2$$

$$\hat{n} \cdot \vec{v}_1 \hat{n} \times \vec{S}_1 \cdot \vec{v}_1 - \frac{144}{35} \log\left(\frac{r}{R_\theta}\right) \vec{v}_1 \cdot \vec{v}_1 \hat{n} \times \vec{S}_1 \cdot \vec{v}_1 - \frac{24}{5} \log\left(\frac{r}{R_\theta}\right) \vec{v}_1 \cdot \vec{v}_2 \hat{n} \times \vec{S}_1 \cdot \vec{v}_1 - \frac{1200}{49} (\hat{n} \cdot \vec{v}_1)^2 \hat{n} \times \vec{S}_1 \cdot \vec{v}_1 +$$

$$\left. \frac{116}{25} \hat{n} \cdot \vec{v}_1 \vec{S}_1 \times \vec{v}_1 \cdot \vec{v}_2 - 28 \hat{n} \cdot \vec{v}_2 \hat{n} \cdot \vec{v}_1 \hat{n} \times \vec{S}_1 \cdot \vec{v}_1 + \frac{6252 \vec{v}_1 \cdot \vec{v}_1 \hat{n} \times \vec{S}_1 \cdot \vec{v}_1}{1225} + \frac{116}{25} \vec{v}_1 \cdot \vec{v}_2 \hat{n} \times \vec{S}_1 \cdot \vec{v}_1 \right) \}$$

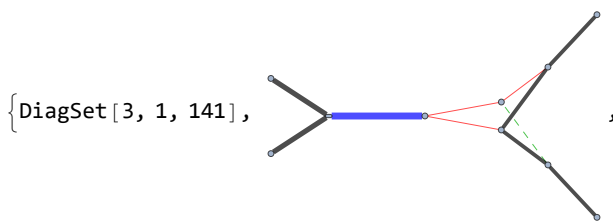

$$\frac{1}{r^3} G^3 \left( 2 \log\left(\frac{r}{R_\theta}\right) \frac{1}{\vec{S}_1 \times \vec{v}_1 \cdot \vec{v}_2} - \frac{1}{\vec{S}_1 \times \vec{v}_1 \cdot \vec{v}_2} + \vec{a}_1 \times \vec{S}_1 \cdot \vec{v}_2 - \frac{9}{25} \hat{n} \times \vec{S}_1 \cdot \vec{v}_2 \hat{n} \cdot \vec{a}_1 - \frac{9}{25} \hat{n} \times \vec{S}_1 \cdot \vec{v}_2 \hat{n} \cdot \vec{v}_1 + \right.$$

$$\left. \frac{116}{25} \hat{n} \times \vec{S}_1 \cdot \vec{v}_1 \hat{n} \cdot \vec{v}_2 - \frac{116}{25} \hat{n} \times \vec{a}_1 \cdot \vec{S}_1 \hat{n} \cdot \vec{v}_2 - 2 \vec{a}_1 \times \vec{S}_1 \cdot \vec{v}_2 \log\left(\frac{r}{R_\theta}\right) + \frac{6}{5} \hat{n} \times \vec{S}_1 \cdot \vec{v}_2 \hat{n} \cdot \vec{a}_1 \log\left(\frac{r}{R_\theta}\right) + \right.$$

$$\left. \frac{6}{5} \hat{n} \times \vec{S}_1 \cdot \vec{v}_2 \hat{n} \cdot \vec{v}_1 \log\left(\frac{r}{R_\theta}\right) - \frac{24}{5} \hat{n} \times \vec{S}_1 \cdot \vec{v}_1 \hat{n} \cdot \vec{v}_2 \log\left(\frac{r}{R_\theta}\right) + \frac{24}{5} \hat{n} \times \vec{a}_1 \cdot \vec{S}_1 \hat{n} \cdot \vec{v}_2 \log\left(\frac{r}{R_\theta}\right) + \frac{1}{\epsilon_d} \right.$$

$$\left. \left( -\frac{2}{3} \frac{1}{\vec{S}_1 \times \vec{v}_1 \cdot \vec{v}_2} + \frac{2}{3} \vec{a}_1 \times \vec{S}_1 \cdot \vec{v}_2 - \frac{2}{5} \hat{n} \times \vec{S}_1 \cdot \vec{v}_2 \hat{n} \cdot \vec{a}_1 - \frac{2}{5} \hat{n} \times \vec{S}_1 \cdot \vec{v}_2 \hat{n} \cdot \vec{v}_1 + \frac{8}{5} \hat{n} \times \vec{S}_1 \cdot \vec{v}_1 \hat{n} \cdot \vec{v}_2 - \frac{8}{5} \hat{n} \times \vec{a}_1 \cdot \vec{S}_1 \hat{n} \cdot \vec{v}_2 \right) \right)$$

$$m_2^3 + \frac{1}{r^4} G^3 \left( 3 \hat{n} \times \vec{S}_1 \cdot \vec{v}_2 (\hat{n} \cdot \vec{v}_1)^2 - 6 \hat{n} \times \vec{S}_1 \cdot \vec{v}_2 \log\left(\frac{r}{R_\theta}\right) (\hat{n} \cdot \vec{v}_1)^2 + \frac{134}{25} \vec{S}_1 \times \vec{v}_1 \cdot \vec{v}_2 \hat{n} \cdot \vec{v}_1 - 28 \hat{n} \times \vec{S}_1 \cdot \vec{v}_1 \hat{n} \cdot \vec{v}_2 \hat{n} \cdot \vec{v}_1 - \right.$$

$$\frac{603}{49} \hat{n} \times \vec{S}_1 \cdot \vec{v}_2 \hat{n} \cdot \vec{v}_2 \hat{n} \cdot \vec{v}_1 - \frac{36}{5} \vec{S}_1 \times \vec{v}_1 \cdot \vec{v}_2 \log\left(\frac{r}{R_\theta}\right) \hat{n} \cdot \vec{v}_1 + 24 \hat{n} \times \vec{S}_1 \cdot \vec{v}_1 \hat{n} \cdot \vec{v}_2 \log\left(\frac{r}{R_\theta}\right) \hat{n} \cdot \vec{v}_1 +$$

$$\frac{90}{7} \hat{n} \times \vec{S}_1 \cdot \vec{v}_2 \hat{n} \cdot \vec{v}_2 \log\left(\frac{r}{R_\theta}\right) \hat{n} \cdot \vec{v}_1 - \frac{228}{49} \hat{n} \times \vec{S}_1 \cdot \vec{v}_1 (\hat{n} \cdot \vec{v}_2)^2 - \frac{9}{25} \vec{S}_1 \times \vec{v}_1 \cdot \vec{v}_2 \hat{n} \cdot \vec{v}_2 - \frac{9}{25} \hat{n} \times \vec{S}_1 \cdot \vec{v}_2 \vec{v}_1 \cdot \vec{v}_1 +$$

$$\frac{116}{25} \hat{n} \times \vec{S}_1 \cdot \vec{v}_1 \vec{v}_1 \cdot \vec{v}_2 + \frac{1149}{245} \hat{n} \times \vec{S}_1 \cdot \vec{v}_2 \vec{v}_1 \cdot \vec{v}_2 + \frac{2652 \hat{n} \times \vec{S}_1 \cdot \vec{v}_1 \vec{v}_2 \cdot \vec{v}_2}{1225} + \frac{24}{7} \hat{n} \times \vec{S}_1 \cdot \vec{v}_1 (\hat{n} \cdot \vec{v}_2)^2 \log\left(\frac{r}{R_\theta}\right) +$$

$$\frac{6}{5} \vec{S}_1 \times \vec{v}_1 \cdot \vec{v}_2 \hat{n} \cdot \vec{v}_2 \log\left(\frac{r}{R_\theta}\right) + \frac{6}{5} \hat{n} \times \vec{S}_1 \cdot \vec{v}_2 \vec{v}_1 \cdot \vec{v}_1 \log\left(\frac{r}{R_\theta}\right) - \frac{24}{5} \hat{n} \times \vec{S}_1 \cdot \vec{v}_1 \vec{v}_1 \cdot \vec{v}_2 \log\left(\frac{r}{R_\theta}\right) -$$

$$\frac{18}{7} \hat{n} \times \vec{S}_1 \cdot \vec{v}_2 \vec{v}_1 \cdot \vec{v}_2 \log\left(\frac{r}{R_\theta}\right) - \frac{24}{35} \hat{n} \times \vec{S}_1 \cdot \vec{v}_1 \vec{v}_2 \cdot \vec{v}_2 \log\left(\frac{r}{R_\theta}\right) + \frac{1}{\epsilon_d} \left( 2 \hat{n} \times \vec{S}_1 \cdot \vec{v}_2 (\hat{n} \cdot \vec{v}_1)^2 + \frac{12}{5} \vec{S}_1 \times \vec{v}_1 \cdot \vec{v}_2 \hat{n} \cdot \vec{v}_1 - \right.$$

$$\left. 8 \hat{n} \times \vec{S}_1 \cdot \vec{v}_1 \hat{n} \cdot \vec{v}_2 \hat{n} \cdot \vec{v}_1 - \frac{30}{7} \hat{n} \times \vec{S}_1 \cdot \vec{v}_2 \hat{n} \cdot \vec{v}_2 \hat{n} \cdot \vec{v}_1 - \frac{8}{7} \hat{n} \times \vec{S}_1 \cdot \vec{v}_1 (\hat{n} \cdot \vec{v}_2)^2 - \frac{2}{5} \vec{S}_1 \times \vec{v}_1 \cdot \vec{v}_2 \hat{n} \cdot \vec{v}_2 - \right.$$

$$\left. \frac{2}{5} \hat{n} \times \vec{S}_1 \cdot \vec{v}_2 \vec{v}_1 \cdot \vec{v}_1 + \frac{8}{5} \hat{n} \times \vec{S}_1 \cdot \vec{v}_1 \vec{v}_1 \cdot \vec{v}_2 + \frac{6}{7} \hat{n} \times \vec{S}_1 \cdot \vec{v}_2 \vec{v}_1 \cdot \vec{v}_2 + \frac{8}{35} \hat{n} \times \vec{S}_1 \cdot \vec{v}_1 \vec{v}_2 \cdot \vec{v}_2 \right) m_2^3 \}$$

{DiagSet[3, 1, 142],

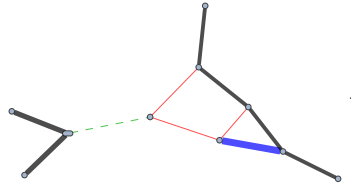

$$\frac{1}{r^3} G^3 m_2^3 \left( \frac{\frac{8}{5} \hat{n} \cdot \vec{v}_2 \hat{n} \times \vec{a}_2 \cdot \vec{S}_1 - \frac{8}{5} \hat{n} \cdot \vec{a}_2 \hat{n} \times \vec{S}_1 \cdot \vec{v}_2}{\epsilon_d} + \frac{24}{5} \log\left(\frac{r}{R_\theta}\right) \hat{n} \cdot \vec{a}_2 \hat{n} \times \vec{S}_1 \cdot \vec{v}_2 - \right.$$

$$\left. \frac{24}{5} \log\left(\frac{r}{R_\theta}\right) \hat{n} \cdot \vec{v}_2 \hat{n} \times \vec{a}_2 \cdot \vec{S}_1 - \frac{116}{25} \hat{n} \cdot \vec{a}_2 \hat{n} \times \vec{S}_1 \cdot \vec{v}_2 + \frac{116}{25} \hat{n} \cdot \vec{v}_2 \hat{n} \times \vec{a}_2 \cdot \vec{S}_1 \right) +$$

$$\frac{1}{r^4} G^3 m_2^3 \left( \frac{\frac{8}{7} \vec{v}_2 \cdot \vec{v}_2 \hat{n} \times \vec{S}_1 \cdot \vec{v}_2 - \frac{40}{7} (\hat{n} \cdot \vec{v}_2)^2 \hat{n} \times \vec{S}_1 \cdot \vec{v}_2}{\epsilon_d} + \frac{120}{7} \log\left(\frac{r}{R_\theta}\right) (\hat{n} \cdot \vec{v}_2)^2 \hat{n} \times \vec{S}_1 \cdot \vec{v}_2 - \right.$$

$$\left. \frac{24}{7} \log\left(\frac{r}{R_\theta}\right) \vec{v}_2 \cdot \vec{v}_2 \hat{n} \times \vec{S}_1 \cdot \vec{v}_2 - \frac{1028}{49} (\hat{n} \cdot \vec{v}_2)^2 \hat{n} \times \vec{S}_1 \cdot \vec{v}_2 + \frac{1364}{245} \vec{v}_2 \cdot \vec{v}_2 \hat{n} \times \vec{S}_1 \cdot \vec{v}_2 \right\}$$

{DiagSet[3, 1, 143],

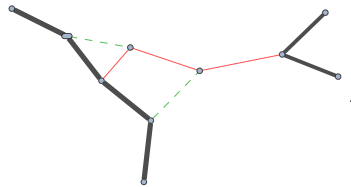

$$\frac{1}{r^3} G^3 m_1^2 m_2 \left( \frac{\hat{n} \cdot \vec{v}_1 \hat{n} \times \vec{S}_1 \cdot \vec{a}_1 + \frac{1}{3} \vec{S}_1 \times \vec{v}_1 \cdot \vec{a}_1 + \hat{n} \cdot \vec{v}_1 \hat{n} \times \vec{S}_1 \cdot \vec{v}_1}{\epsilon_d} - 3 \log\left(\frac{r}{R_\theta}\right) \hat{n} \cdot \vec{v}_1 \hat{n} \times \vec{S}_1 \cdot \vec{a}_1 + \right.$$

$$\left. \hat{n} \cdot \vec{v}_1 \hat{n} \times \vec{S}_1 \cdot \vec{a}_1 - \log\left(\frac{r}{R_\theta}\right) \vec{S}_1 \times \vec{v}_1 \cdot \vec{a}_1 - 3 \log\left(\frac{r}{R_\theta}\right) \hat{n} \cdot \vec{v}_1 \hat{n} \times \vec{S}_1 \cdot \vec{v}_1 + \hat{n} \cdot \vec{v}_1 \hat{n} \times \vec{S}_1 \cdot \vec{v}_1 \right) + \frac{1}{r^4}$$

$$G^3 m_1^2 m_2 \left( \frac{1}{\epsilon_d} \left( -4 (\hat{n} \cdot \vec{v}_1)^2 \hat{n} \times \vec{S}_1 \cdot \vec{v}_1 + \frac{4}{5} \hat{n} \cdot \vec{v}_1 \vec{S}_1 \times \vec{v}_1 \cdot \vec{v}_2 - 4 \hat{n} \cdot \vec{v}_2 \hat{n} \cdot \vec{v}_1 \hat{n} \times \vec{S}_1 \cdot \vec{v}_1 + \frac{4}{5} \vec{v}_1 \cdot \vec{v}_1 \hat{n} \times \vec{S}_1 \cdot \vec{v}_1 + \right. \right.$$

$$\left. \frac{4}{5} \vec{v}_1 \cdot \vec{v}_2 \hat{n} \times \vec{S}_1 \cdot \vec{v}_1 \right) + 12 \log\left(\frac{r}{R_\theta}\right) (\hat{n} \cdot \vec{v}_1)^2 \hat{n} \times \vec{S}_1 \cdot \vec{v}_1 - \frac{12}{5} \log\left(\frac{r}{R_\theta}\right) \hat{n} \cdot \vec{v}_1 \vec{S}_1 \times \vec{v}_1 \cdot \vec{v}_2 +$$

$$12 \log\left(\frac{r}{R_\theta}\right) \hat{n} \cdot \vec{v}_2 \hat{n} \cdot \vec{v}_1 \hat{n} \times \vec{S}_1 \cdot \vec{v}_1 - \frac{12}{5} \log\left(\frac{r}{R_\theta}\right) \vec{v}_1 \cdot \vec{v}_1 \hat{n} \times \vec{S}_1 \cdot \vec{v}_1 - \frac{12}{5} \log\left(\frac{r}{R_\theta}\right) \vec{v}_1 \cdot \vec{v}_2 \hat{n} \times \vec{S}_1 \cdot \vec{v}_1 -$$

$$6 (\hat{n} \cdot \vec{v}_1)^2 \hat{n} \times \vec{S}_1 \cdot \vec{v}_1 + \frac{18}{25} \hat{n} \cdot \vec{v}_1 \vec{S}_1 \times \vec{v}_1 \cdot \vec{v}_2 - 6 \hat{n} \cdot \vec{v}_2 \hat{n} \cdot \vec{v}_1 \hat{n} \times \vec{S}_1 \cdot \vec{v}_1 + \frac{18}{25} \vec{v}_1 \cdot \vec{v}_1 \hat{n} \times \vec{S}_1 \cdot \vec{v}_1 + \frac{18}{25} \vec{v}_1 \cdot \vec{v}_2 \hat{n} \times \vec{S}_1 \cdot \vec{v}_1 \Big\}$$

{DiagSet[3, 1, 144],

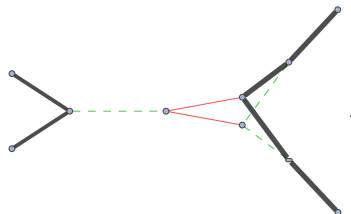

$$\frac{1}{r^3} G^3 m_1^2 m_2 \left( \frac{-\frac{4}{5} \hat{n} \cdot \vec{v}_2 \hat{n} \times \vec{S}_1 \cdot \vec{a}_1 + \frac{4}{15} \vec{S}_1 \times \vec{a}_1 \cdot \vec{v}_2 - \frac{4}{5} \hat{n} \cdot \vec{v}_2 \hat{n} \times \vec{S}_1 \cdot \vec{v}_1 + \frac{4}{15} \vec{S}_1 \times \vec{v}_1 \cdot \vec{v}_2}{\epsilon_d} + \right.$$

$$\begin{aligned} & \frac{12}{5} \log\left(\frac{r}{R_\theta}\right) \hat{n} \cdot \vec{v}_2 \hat{n} \times \vec{S}_1 \cdot \vec{a}_1 - \frac{38}{25} \hat{n} \cdot \vec{v}_2 \hat{n} \times \vec{S}_1 \cdot \vec{a}_1 - \frac{4}{5} \log\left(\frac{r}{R_\theta}\right) \vec{S}_1 \times \vec{a}_1 \cdot \vec{v}_2 - \frac{2}{75} \vec{S}_1 \times \vec{a}_1 \cdot \vec{v}_2 + \\ & \frac{12}{5} \log\left(\frac{r}{R_\theta}\right) \hat{n} \cdot \vec{v}_2 \hat{n} \times \vec{S}_1 \cdot \vec{v}_1 - \frac{38}{25} \hat{n} \cdot \vec{v}_2 \hat{n} \times \vec{S}_1 \cdot \vec{v}_1 - \frac{4}{5} \log\left(\frac{r}{R_\theta}\right) \vec{S}_1 \times \vec{v}_1 \cdot \vec{v}_2 - \frac{2}{75} \vec{S}_1 \times \vec{v}_1 \cdot \vec{v}_2 \Bigg) + \\ & \frac{1}{r^4} G^3 m_1^2 m_2 \left( \frac{-\frac{32}{35} \hat{n} \cdot \vec{v}_1 \vec{S}_1 \times \vec{v}_1 \cdot \vec{v}_2 + \frac{32}{7} \hat{n} \cdot \vec{v}_2 \hat{n} \cdot \vec{v}_1 \hat{n} \times \vec{S}_1 \cdot \vec{v}_1 - \frac{32}{35} \vec{v}_1 \cdot \vec{v}_2 \hat{n} \times \vec{S}_1 \cdot \vec{v}_1}{\epsilon_d} + \right. \\ & \frac{96}{35} \log\left(\frac{r}{R_\theta}\right) \hat{n} \cdot \vec{v}_1 \vec{S}_1 \times \vec{v}_1 \cdot \vec{v}_2 - \frac{96}{7} \log\left(\frac{r}{R_\theta}\right) \hat{n} \cdot \vec{v}_2 \hat{n} \cdot \vec{v}_1 \hat{n} \times \vec{S}_1 \cdot \vec{v}_1 + \frac{96}{35} \log\left(\frac{r}{R_\theta}\right) \vec{v}_1 \cdot \vec{v}_2 \hat{n} \times \vec{S}_1 \cdot \vec{v}_1 - \\ & \left. \frac{2068 \hat{n} \cdot \vec{v}_1 \vec{S}_1 \times \vec{v}_1 \cdot \vec{v}_2}{1225} + \frac{576}{49} \hat{n} \cdot \vec{v}_2 \hat{n} \cdot \vec{v}_1 \hat{n} \times \vec{S}_1 \cdot \vec{v}_1 - \frac{1088 \vec{v}_1 \cdot \vec{v}_2 \hat{n} \times \vec{S}_1 \cdot \vec{v}_1}{1225} \right) \Bigg\} \end{aligned}$$

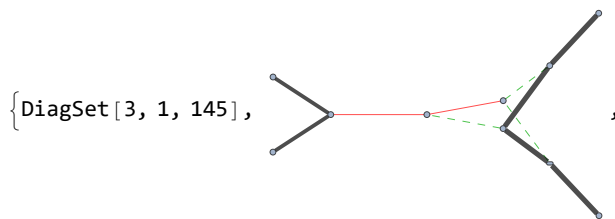

$$\begin{aligned} & \frac{1}{r^3} G^3 m_1^2 m_2 \left( \frac{4 \hat{n} \cdot \vec{v}_1 \hat{n} \times \vec{S}_1 \cdot \vec{a}_1 + \frac{4}{3} \vec{S}_1 \times \vec{v}_1 \cdot \vec{a}_1 + 4 \hat{n} \cdot \vec{v}_1 \hat{n} \times \vec{S}_1 \cdot \vec{v}_1}{\epsilon_d} - 12 \log\left(\frac{r}{R_\theta}\right) \hat{n} \cdot \vec{v}_1 \hat{n} \times \vec{S}_1 \cdot \vec{a}_1 + 6 \hat{n} \cdot \vec{v}_1 \hat{n} \times \vec{S}_1 \cdot \vec{a}_1 - \right. \\ & \left. 4 \log\left(\frac{r}{R_\theta}\right) \vec{S}_1 \times \vec{v}_1 \cdot \vec{a}_1 + \frac{2}{3} \vec{S}_1 \times \vec{v}_1 \cdot \vec{a}_1 - 12 \log\left(\frac{r}{R_\theta}\right) \hat{n} \cdot \vec{v}_1 \hat{n} \times \vec{S}_1 \cdot \vec{v}_1 + 6 \hat{n} \cdot \vec{v}_1 \hat{n} \times \vec{S}_1 \cdot \vec{v}_1 \right) + \frac{1}{r^4} \end{aligned}$$

$$\begin{aligned} & G^3 m_1^2 m_2 \left( \frac{1}{\epsilon_d} \left( -16 (\hat{n} \cdot \vec{v}_1)^2 \hat{n} \times \vec{S}_1 \cdot \vec{v}_1 + \frac{16}{5} \hat{n} \cdot \vec{v}_1 \vec{S}_1 \times \vec{v}_1 \cdot \vec{v}_2 - 16 \hat{n} \cdot \vec{v}_2 \hat{n} \cdot \vec{v}_1 \hat{n} \times \vec{S}_1 \cdot \vec{v}_1 + \frac{16}{5} \vec{v}_1 \cdot \vec{v}_1 \hat{n} \times \vec{S}_1 \cdot \vec{v}_1 + \right. \right. \\ & \frac{16}{5} \vec{v}_1 \cdot \vec{v}_2 \hat{n} \times \vec{S}_1 \cdot \vec{v}_1 \Bigg) + 48 \log\left(\frac{r}{R_\theta}\right) (\hat{n} \cdot \vec{v}_1)^2 \hat{n} \times \vec{S}_1 \cdot \vec{v}_1 - \frac{48}{5} \log\left(\frac{r}{R_\theta}\right) \hat{n} \cdot \vec{v}_1 \vec{S}_1 \times \vec{v}_1 \cdot \vec{v}_2 + 48 \log\left(\frac{r}{R_\theta}\right) \hat{n} \cdot \vec{v}_2 \\ & \hat{n} \cdot \vec{v}_1 \hat{n} \times \vec{S}_1 \cdot \vec{v}_1 - \frac{48}{5} \log\left(\frac{r}{R_\theta}\right) \vec{v}_1 \cdot \vec{v}_1 \hat{n} \times \vec{S}_1 \cdot \vec{v}_1 - \frac{48}{5} \log\left(\frac{r}{R_\theta}\right) \vec{v}_1 \cdot \vec{v}_2 \hat{n} \times \vec{S}_1 \cdot \vec{v}_1 - 32 (\hat{n} \cdot \vec{v}_1)^2 \hat{n} \times \vec{S}_1 \cdot \vec{v}_1 + \\ & \left. \frac{112}{25} \hat{n} \cdot \vec{v}_1 \vec{S}_1 \times \vec{v}_1 \cdot \vec{v}_2 - 32 \hat{n} \cdot \vec{v}_2 \hat{n} \cdot \vec{v}_1 \hat{n} \times \vec{S}_1 \cdot \vec{v}_1 + \frac{112}{25} \vec{v}_1 \cdot \vec{v}_1 \hat{n} \times \vec{S}_1 \cdot \vec{v}_1 + \frac{112}{25} \vec{v}_1 \cdot \vec{v}_2 \hat{n} \times \vec{S}_1 \cdot \vec{v}_1 \right) \Bigg\} \end{aligned}$$

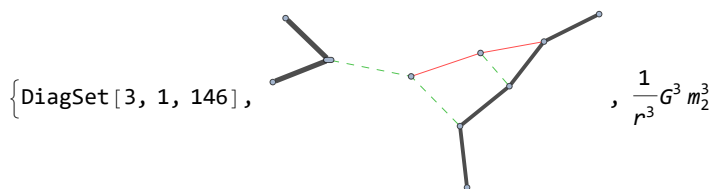

$$\begin{aligned} & \left( \frac{-8 \hat{n} \cdot \vec{a}_2 \hat{n} \times \vec{S}_1 \cdot \vec{v}_2 - 8 \hat{n} \cdot \vec{v}_2 \hat{n} \times \vec{a}_2 \cdot \vec{S}_1 + \frac{16}{3} \vec{a}_2 \times \vec{S}_1 \cdot \vec{v}_2}{\epsilon_d} + 24 \log\left(\frac{r}{R_\theta}\right) \hat{n} \cdot \vec{a}_2 \hat{n} \times \vec{S}_1 \cdot \vec{v}_2 + 24 \log\left(\frac{r}{R_\theta}\right) \hat{n} \cdot \vec{v}_2 \hat{n} \times \vec{a}_2 \cdot \vec{S}_1 - \right. \\ & \left. 16 \hat{n} \cdot \vec{a}_2 \hat{n} \times \vec{S}_1 \cdot \vec{v}_2 - 32 \hat{n} \cdot \vec{v}_2 \hat{n} \times \vec{a}_2 \cdot \vec{S}_1 - 16 \log\left(\frac{r}{R_\theta}\right) \vec{a}_2 \times \vec{S}_1 \cdot \vec{v}_2 + \frac{32}{3} \vec{a}_2 \times \vec{S}_1 \cdot \vec{v}_2 + 16 \hat{n} \cdot \vec{v}_2 \hat{n} \times \vec{S}_1 \cdot \vec{v}_2 \right) + \frac{1}{r^4} G^3 m_2^3 \\ & \left( 16 (\hat{n} \cdot \vec{v}_2)^2 \hat{n} \times \vec{S}_1 \cdot \vec{v}_2 - 16 \hat{n} \cdot \vec{v}_2 \vec{S}_1 \times \vec{v}_1 \cdot \vec{v}_2 - 80 \hat{n} \cdot \vec{v}_1 \hat{n} \cdot \vec{v}_2 \hat{n} \times \vec{S}_1 \cdot \vec{v}_2 + 16 \vec{v}_1 \cdot \vec{v}_2 \hat{n} \times \vec{S}_1 \cdot \vec{v}_2 + 16 \vec{v}_2 \cdot \vec{v}_2 \hat{n} \times \vec{S}_1 \cdot \vec{v}_2 \right) \Bigg\} \end{aligned}$$

{DiagSet[3, 1, 147],

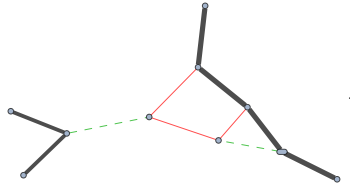

$$\frac{1}{r^3} G^3 m_1^2 m_2 \left( \frac{-\frac{1}{5} \hat{n} \cdot \vec{v}_2 \hat{n} \times \vec{S}_1 \cdot \vec{a}_1 + \frac{1}{15} \vec{S}_1 \times \vec{a}_1 \cdot \vec{v}_2 - \frac{1}{5} \hat{n} \cdot \vec{v}_2 \hat{n} \times \vec{S}_1 \cdot \vec{v}_1 + \frac{1}{15} \vec{S}_1 \times \vec{v}_1 \cdot \vec{v}_2}{\epsilon_d} + \right.$$

$$\frac{3}{5} \log\left(\frac{r}{R_\theta}\right) \hat{n} \cdot \vec{v}_2 \hat{n} \times \vec{S}_1 \cdot \vec{a}_1 - \frac{7}{25} \hat{n} \cdot \vec{v}_2 \hat{n} \times \vec{S}_1 \cdot \vec{a}_1 - \frac{1}{5} \log\left(\frac{r}{R_\theta}\right) \vec{S}_1 \times \vec{a}_1 \cdot \vec{v}_2 - \frac{1}{25} \vec{S}_1 \times \vec{a}_1 \cdot \vec{v}_2 +$$

$$\frac{3}{5} \log\left(\frac{r}{R_\theta}\right) \hat{n} \cdot \vec{v}_2 \hat{n} \times \vec{S}_1 \cdot \vec{v}_1 - \frac{7}{25} \hat{n} \cdot \vec{v}_2 \hat{n} \times \vec{S}_1 \cdot \vec{v}_1 - \frac{1}{5} \log\left(\frac{r}{R_\theta}\right) \vec{S}_1 \times \vec{v}_1 \cdot \vec{v}_2 - \frac{1}{25} \vec{S}_1 \times \vec{v}_1 \cdot \vec{v}_2 \left. \right) +$$

$$\frac{1}{r^4} G^3 m_1^2 m_2 \left( \frac{-\frac{8}{35} \hat{n} \cdot \vec{v}_1 \vec{S}_1 \times \vec{v}_1 \cdot \vec{v}_2 + \frac{8}{7} \hat{n} \cdot \vec{v}_2 \hat{n} \cdot \vec{v}_1 \hat{n} \times \vec{S}_1 \cdot \vec{v}_1 - \frac{8}{35} \vec{v}_1 \cdot \vec{v}_2 \hat{n} \times \vec{S}_1 \cdot \vec{v}_1}{\epsilon_d} + \right.$$

$$\frac{24}{35} \log\left(\frac{r}{R_\theta}\right) \hat{n} \cdot \vec{v}_1 \vec{S}_1 \times \vec{v}_1 \cdot \vec{v}_2 - \frac{24}{7} \log\left(\frac{r}{R_\theta}\right) \hat{n} \cdot \vec{v}_2 \hat{n} \cdot \vec{v}_1 \hat{n} \times \vec{S}_1 \cdot \vec{v}_1 + \frac{24}{35} \log\left(\frac{r}{R_\theta}\right) \vec{v}_1 \cdot \vec{v}_2 \hat{n} \times \vec{S}_1 \cdot \vec{v}_1 -$$

$$\left. \frac{377 \hat{n} \cdot \vec{v}_1 \vec{S}_1 \times \vec{v}_1 \cdot \vec{v}_2}{1225} + \frac{116}{49} \hat{n} \cdot \vec{v}_2 \hat{n} \cdot \vec{v}_1 \hat{n} \times \vec{S}_1 \cdot \vec{v}_1 - \frac{132 \vec{v}_1 \cdot \vec{v}_2 \hat{n} \times \vec{S}_1 \cdot \vec{v}_1}{1225} \right\}$$

{DiagSet[3, 1, 148],

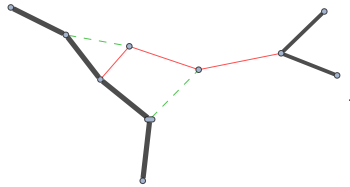

$$\frac{m_1^2 m_2 \left( 2 \log\left(\frac{r}{R_\theta}\right) \hat{n} \times \vec{S}_1 \cdot \vec{a}_1 - \frac{2 \hat{n} \times \vec{S}_1 \cdot \vec{a}_1}{3 \epsilon_d} - \hat{n} \times \vec{S}_1 \cdot \vec{a}_1 \right) G^3}{r^2} + \frac{1}{r^3} m_1^2 m_2$$

$$\left( 2 \log\left(\frac{r}{R_\theta}\right) \vec{S}_1 \times \vec{v}_1 \cdot \vec{v}_2 - \vec{S}_1 \times \vec{v}_1 \cdot \vec{v}_2 + \vec{S}_1 \times \vec{a}_1 \cdot \vec{v}_2 + \vec{S}_1 \times \vec{v}_1 \cdot \vec{a}_1 - \vec{S}_1 \times \vec{v}_1 \cdot \vec{a}_2 - \frac{174}{25} \hat{n} \times \vec{S}_1 \cdot \vec{v}_1 \hat{n} \cdot \vec{a}_1 + 5 \hat{n} \times \vec{S}_1 \cdot \vec{v}_1 \hat{n} \cdot \vec{a}_2 + \right.$$

$$\frac{116}{25} \hat{n} \times \vec{S}_1 \cdot \vec{v}_1 \hat{n} \cdot \vec{v}_1 - \frac{49}{25} \hat{n} \times \vec{S}_1 \cdot \vec{a}_1 \hat{n} \cdot \vec{v}_1 + 5 \hat{n} \times \vec{S}_1 \cdot \vec{v}_1 \hat{n} \cdot \vec{v}_2 - 5 \hat{n} \times \vec{S}_1 \cdot \vec{a}_1 \hat{n} \cdot \vec{v}_2 - 2 \vec{S}_1 \times \vec{a}_1 \cdot \vec{v}_2 \log\left(\frac{r}{R_\theta}\right) -$$

$$2 \vec{S}_1 \times \vec{v}_1 \cdot \vec{a}_1 \log\left(\frac{r}{R_\theta}\right) + 2 \vec{S}_1 \times \vec{v}_1 \cdot \vec{a}_2 \log\left(\frac{r}{R_\theta}\right) + \frac{36}{5} \hat{n} \times \vec{S}_1 \cdot \vec{v}_1 \hat{n} \cdot \vec{a}_1 \log\left(\frac{r}{R_\theta}\right) - 6 \hat{n} \times \vec{S}_1 \cdot \vec{v}_1 \hat{n} \cdot \vec{a}_2 \log\left(\frac{r}{R_\theta}\right) -$$

$$\frac{24}{5} \hat{n} \times \vec{S}_1 \cdot \vec{v}_1 \hat{n} \cdot \vec{v}_1 \log\left(\frac{r}{R_\theta}\right) + \frac{6}{5} \hat{n} \times \vec{S}_1 \cdot \vec{a}_1 \hat{n} \cdot \vec{v}_1 \log\left(\frac{r}{R_\theta}\right) - 6 \hat{n} \times \vec{S}_1 \cdot \vec{v}_1 \hat{n} \cdot \vec{v}_2 \log\left(\frac{r}{R_\theta}\right) + 6 \hat{n} \times \vec{S}_1 \cdot \vec{a}_1$$

$$\hat{n} \cdot \vec{v}_2 \log\left(\frac{r}{R_\theta}\right) + \frac{1}{\epsilon_d} \left( -\frac{2}{3} \vec{S}_1 \times \vec{v}_1 \cdot \vec{v}_2 + \frac{2}{3} \vec{S}_1 \times \vec{a}_1 \cdot \vec{v}_2 + \frac{2}{3} \vec{S}_1 \times \vec{v}_1 \cdot \vec{a}_1 - \frac{2}{3} \vec{S}_1 \times \vec{v}_1 \cdot \vec{a}_2 - \frac{12}{5} \hat{n} \times \vec{S}_1 \cdot \vec{v}_1 \hat{n} \cdot \vec{a}_1 + \right.$$

$$\left. 2 \hat{n} \times \vec{S}_1 \cdot \vec{v}_1 \hat{n} \cdot \vec{a}_2 + \frac{8}{5} \hat{n} \times \vec{S}_1 \cdot \vec{v}_1 \hat{n} \cdot \vec{v}_1 - \frac{2}{5} \hat{n} \times \vec{S}_1 \cdot \vec{a}_1 \hat{n} \cdot \vec{v}_1 + 2 \hat{n} \times \vec{S}_1 \cdot \vec{v}_1 \hat{n} \cdot \vec{v}_2 - 2 \hat{n} \times \vec{S}_1 \cdot \vec{a}_1 \hat{n} \cdot \vec{v}_2 \right) \left. \right) G^3 + \frac{1}{r^4}$$

$$m_1^2 m_2 \left( \frac{1028}{49} \hat{n} \times \vec{S}_1 \cdot \vec{v}_1 (\hat{n} \cdot \vec{v}_1)^2 - \frac{120}{7} \hat{n} \times \vec{S}_1 \cdot \vec{v}_1 \log\left(\frac{r}{R_\theta}\right) (\hat{n} \cdot \vec{v}_1)^2 - \frac{223}{25} \vec{S}_1 \times \vec{v}_1 \cdot \vec{v}_2 \hat{n} \cdot \vec{v}_1 + 53 \hat{n} \times \vec{S}_1 \cdot \vec{v}_1 \hat{n} \cdot \vec{v}_2 \hat{n} \cdot \vec{v}_1 + \right.$$

$$\frac{42}{5} \vec{S}_1 \times \vec{v}_1 \cdot \vec{v}_2 \log\left(\frac{r}{R_\theta}\right) \hat{n} \cdot \vec{v}_1 - 42 \hat{n} \times \vec{S}_1 \cdot \vec{v}_1 \hat{n} \cdot \vec{v}_2 \log\left(\frac{r}{R_\theta}\right) \hat{n} \cdot \vec{v}_1 + 31 \hat{n} \times \vec{S}_1 \cdot \vec{v}_1 (\hat{n} \cdot \vec{v}_2)^2 - 10 \vec{S}_1 \times \vec{v}_1 \cdot \vec{v}_2 \hat{n} \cdot \vec{v}_2 -$$

$$\left. \frac{1364}{245} \hat{n} \times \vec{S}_1 \cdot \vec{v}_1 \vec{v}_1 \cdot \vec{v}_1 - \frac{223}{25} \hat{n} \times \vec{S}_1 \cdot \vec{v}_1 \vec{v}_1 \cdot \vec{v}_2 - 5 \hat{n} \times \vec{S}_1 \cdot \vec{v}_1 \vec{v}_2 \cdot \vec{v}_2 - 30 \hat{n} \times \vec{S}_1 \cdot \vec{v}_1 (\hat{n} \cdot \vec{v}_2)^2 \log\left(\frac{r}{R_\theta}\right) + \right.$$



$$\begin{aligned} & 12 \vec{S}_1 \times \vec{v}_1 \cdot \vec{v}_2 \hat{n} \cdot \vec{v}_2 \log\left(\frac{r}{R_\theta}\right) + \frac{24}{7} \hat{n} \times \vec{S}_1 \cdot \vec{v}_1 \vec{v}_1 \cdot \vec{v}_1 \log\left(\frac{r}{R_\theta}\right) + \frac{42}{5} \hat{n} \times \vec{S}_1 \cdot \vec{v}_1 \vec{v}_1 \cdot \vec{v}_2 \log\left(\frac{r}{R_\theta}\right) + \\ & 6 \hat{n} \times \vec{S}_1 \cdot \vec{v}_1 \vec{v}_2 \cdot \vec{v}_2 \log\left(\frac{r}{R_\theta}\right) + \frac{1}{\epsilon_d} \left( \frac{40}{7} \hat{n} \times \vec{S}_1 \cdot \vec{v}_1 (\hat{n} \cdot \vec{v}_1)^2 - \frac{14}{5} \vec{S}_1 \times \vec{v}_1 \cdot \vec{v}_2 \hat{n} \cdot \vec{v}_1 + 14 \hat{n} \times \vec{S}_1 \cdot \vec{v}_1 \hat{n} \cdot \vec{v}_2 \hat{n} \cdot \vec{v}_1 + \right. \\ & \left. 10 \hat{n} \times \vec{S}_1 \cdot \vec{v}_1 (\hat{n} \cdot \vec{v}_2)^2 - 4 \vec{S}_1 \times \vec{v}_1 \cdot \vec{v}_2 \hat{n} \cdot \vec{v}_2 - \frac{8}{7} \hat{n} \times \vec{S}_1 \cdot \vec{v}_1 \vec{v}_1 \cdot \vec{v}_1 - \frac{14}{5} \hat{n} \times \vec{S}_1 \cdot \vec{v}_1 \vec{v}_1 \cdot \vec{v}_2 - 2 \hat{n} \times \vec{S}_1 \cdot \vec{v}_1 \vec{v}_2 \cdot \vec{v}_2 \right) \Big) G^3 \Big\} \end{aligned}$$

{DiagSet[3, 1, 149],

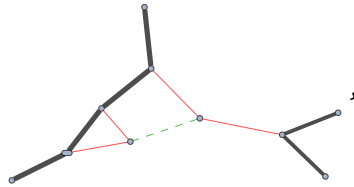

$$\begin{aligned} & \frac{1}{r^3} G^3 m_1^2 m_2 \left( \frac{-\frac{3}{5} \hat{n} \cdot \vec{v}_1 \hat{n} \times \vec{S}_1 \cdot \vec{a}_1 - \frac{1}{5} \vec{S}_1 \times \vec{v}_1 \cdot \vec{a}_1 - \frac{3}{5} \hat{n} \cdot \vec{v}_1 \hat{n} \times \vec{S}_1 \cdot \vec{v}_1}{\epsilon_d} + \frac{9}{5} \log\left(\frac{r}{R_\theta}\right) \hat{n} \cdot \vec{v}_1 \hat{n} \times \vec{S}_1 \cdot \vec{a}_1 - \right. \\ & \frac{6}{25} \hat{n} \cdot \vec{v}_1 \hat{n} \times \vec{S}_1 \cdot \vec{a}_1 + 2 \hat{n} \cdot \vec{v}_2 \hat{n} \times \vec{S}_1 \cdot \vec{a}_1 + \frac{3}{5} \log\left(\frac{r}{R_\theta}\right) \vec{S}_1 \times \vec{v}_1 \cdot \vec{a}_1 - \frac{2}{3} \vec{S}_1 \times \vec{a}_1 \cdot \vec{v}_2 - \frac{1}{75} \vec{S}_1 \times \vec{v}_1 \cdot \vec{a}_1 + \\ & \left. \frac{9}{5} \log\left(\frac{r}{R_\theta}\right) \hat{n} \cdot \vec{v}_1 \hat{n} \times \vec{S}_1 \cdot \vec{v}_1 - \frac{6}{25} \hat{n} \cdot \vec{v}_1 \hat{n} \times \vec{S}_1 \cdot \vec{v}_1 + 2 \hat{n} \cdot \vec{v}_2 \hat{n} \times \vec{S}_1 \cdot \vec{v}_1 - \frac{2}{3} \frac{1}{\vec{S}_1 \times \vec{v}_1 \cdot \vec{v}_2} \right) + \frac{1}{r^4} G^3 m_1^2 m_2 \\ & \left( \frac{1}{\epsilon_d} \left( \frac{9}{7} (\hat{n} \cdot \vec{v}_1)^2 \hat{n} \times \vec{S}_1 \cdot \vec{v}_1 + \frac{1}{5} \hat{n} \cdot \vec{v}_1 \vec{S}_1 \times \vec{v}_1 \cdot \vec{v}_2 - \hat{n} \cdot \vec{v}_2 \hat{n} \cdot \vec{v}_1 \hat{n} \times \vec{S}_1 \cdot \vec{v}_1 - \frac{9}{35} \vec{v}_1 \cdot \vec{v}_1 \hat{n} \times \vec{S}_1 \cdot \vec{v}_1 + \frac{1}{5} \vec{v}_1 \cdot \vec{v}_2 \hat{n} \times \vec{S}_1 \cdot \vec{v}_1 \right) - \right. \\ & \frac{27}{7} \log\left(\frac{r}{R_\theta}\right) (\hat{n} \cdot \vec{v}_1)^2 \hat{n} \times \vec{S}_1 \cdot \vec{v}_1 - \frac{3}{5} \log\left(\frac{r}{R_\theta}\right) \hat{n} \cdot \vec{v}_1 \vec{S}_1 \times \vec{v}_1 \cdot \vec{v}_2 + 3 \log\left(\frac{r}{R_\theta}\right) \hat{n} \cdot \vec{v}_2 \hat{n} \cdot \vec{v}_1 \hat{n} \times \vec{S}_1 \cdot \vec{v}_1 + \\ & \frac{27}{35} \log\left(\frac{r}{R_\theta}\right) \vec{v}_1 \cdot \vec{v}_1 \hat{n} \times \vec{S}_1 \cdot \vec{v}_1 - \frac{3}{5} \log\left(\frac{r}{R_\theta}\right) \vec{v}_1 \cdot \vec{v}_2 \hat{n} \times \vec{S}_1 \cdot \vec{v}_1 + \frac{92}{49} (\hat{n} \cdot \vec{v}_1)^2 \hat{n} \times \vec{S}_1 \cdot \vec{v}_1 + \\ & \left. \frac{37}{25} \hat{n} \cdot \vec{v}_1 \vec{S}_1 \times \vec{v}_1 \cdot \vec{v}_2 - 8 \hat{n} \cdot \vec{v}_2 \hat{n} \cdot \vec{v}_1 \hat{n} \times \vec{S}_1 \cdot \vec{v}_1 - \frac{446 \vec{v}_1 \cdot \vec{v}_1 \hat{n} \times \vec{S}_1 \cdot \vec{v}_1}{1225} + \frac{37}{25} \vec{v}_1 \cdot \vec{v}_2 \hat{n} \times \vec{S}_1 \cdot \vec{v}_1 \right) \Big\} \end{aligned}$$

{DiagSet[3, 1, 150],

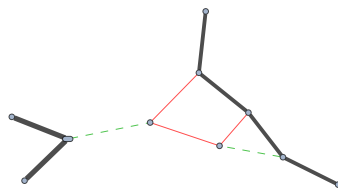

$$\begin{aligned} & G^3 \left( -2 \log\left(\frac{r}{R_\theta}\right) \hat{n} \times \vec{a}_2 \cdot \vec{S}_1 + \frac{2 \hat{n} \times \vec{a}_2 \cdot \vec{S}_1}{3 \epsilon_d} + \hat{n} \times \vec{a}_2 \cdot \vec{S}_1 \right) m_2^3 \\ & \frac{1}{r^2} + \\ & \frac{1}{r^3} G^3 \left( -2 \log\left(\frac{r}{R_\theta}\right) \vec{a}_2 \times \vec{S}_1 \cdot \vec{v}_1 + \vec{a}_2 \times \vec{S}_1 \cdot \vec{v}_1 - 2 \vec{a}_2 \times \vec{S}_1 \cdot \vec{v}_2 + \frac{241}{25} \hat{n} \times \vec{S}_1 \cdot \vec{v}_2 \hat{n} \cdot \vec{a}_2 - 5 \hat{n} \times \vec{a}_2 \cdot \vec{S}_1 \hat{n} \cdot \vec{v}_1 - \right. \\ & \frac{107}{25} \hat{n} \times \vec{S}_1 \cdot \vec{v}_2 \hat{n} \cdot \vec{v}_2 + \frac{9}{25} \hat{n} \times \vec{a}_2 \cdot \vec{S}_1 \hat{n} \cdot \vec{v}_2 + 4 \vec{a}_2 \times \vec{S}_1 \cdot \vec{v}_2 \log\left(\frac{r}{R_\theta}\right) - \frac{54}{5} \hat{n} \times \vec{S}_1 \cdot \vec{v}_2 \hat{n} \cdot \vec{a}_2 \log\left(\frac{r}{R_\theta}\right) + \\ & 6 \hat{n} \times \vec{a}_2 \cdot \vec{S}_1 \hat{n} \cdot \vec{v}_1 \log\left(\frac{r}{R_\theta}\right) + \frac{18}{5} \hat{n} \times \vec{S}_1 \cdot \vec{v}_2 \hat{n} \cdot \vec{v}_2 \log\left(\frac{r}{R_\theta}\right) - \frac{6}{5} \hat{n} \times \vec{a}_2 \cdot \vec{S}_1 \hat{n} \cdot \vec{v}_2 \log\left(\frac{r}{R_\theta}\right) + \frac{1}{\epsilon_d} \\ & \left( \frac{2}{3} \vec{a}_2 \times \vec{S}_1 \cdot \vec{v}_1 - \frac{4}{3} \vec{a}_2 \times \vec{S}_1 \cdot \vec{v}_2 + \frac{18}{5} \hat{n} \times \vec{S}_1 \cdot \vec{v}_2 \hat{n} \cdot \vec{a}_2 - 2 \hat{n} \times \vec{a}_2 \cdot \vec{S}_1 \hat{n} \cdot \vec{v}_1 - \frac{6}{5} \hat{n} \times \vec{S}_1 \cdot \vec{v}_2 \hat{n} \cdot \vec{v}_2 + \frac{2}{5} \hat{n} \times \vec{a}_2 \cdot \vec{S}_1 \hat{n} \cdot \vec{v}_2 \right) \Big) \\ & m_2^3 + \frac{1}{r^4} G^3 \left( \frac{831}{49} \hat{n} \times \vec{S}_1 \cdot \vec{v}_2 (\hat{n} \cdot \vec{v}_2)^2 - \frac{114}{7} \hat{n} \times \vec{S}_1 \cdot \vec{v}_2 \log\left(\frac{r}{R_\theta}\right) (\hat{n} \cdot \vec{v}_2)^2 + \frac{107}{25} \vec{S}_1 \times \vec{v}_1 \cdot \vec{v}_2 \hat{n} \cdot \vec{v}_2 + \right. \\ & \left. 25 \hat{n} \times \vec{S}_1 \cdot \vec{v}_2 \hat{n} \cdot \vec{v}_1 \hat{n} \cdot \vec{v}_2 - \frac{18}{5} \vec{S}_1 \times \vec{v}_1 \cdot \vec{v}_2 \log\left(\frac{r}{R_\theta}\right) \hat{n} \cdot \vec{v}_2 - 18 \hat{n} \times \vec{S}_1 \cdot \vec{v}_2 \hat{n} \cdot \vec{v}_1 \log\left(\frac{r}{R_\theta}\right) \hat{n} \cdot \vec{v}_2 - \right. \end{aligned}$$

$$\frac{107}{25} \hat{n} \times \vec{S}_1 \cdot \vec{v}_2 \vec{v}_1 \cdot \vec{v}_2 - \frac{8397 \hat{n} \times \vec{S}_1 \cdot \vec{v}_2 \vec{v}_2 \cdot \vec{v}_2}{1225} + \frac{18}{5} \hat{n} \times \vec{S}_1 \cdot \vec{v}_2 \vec{v}_1 \cdot \vec{v}_2 \log\left(\frac{r}{R_\theta}\right) +$$

$$\frac{114}{35} \hat{n} \times \vec{S}_1 \cdot \vec{v}_2 \vec{v}_2 \cdot \vec{v}_2 \log\left(\frac{r}{R_\theta}\right) + \frac{1}{\epsilon_d} \left( \frac{38}{7} \hat{n} \times \vec{S}_1 \cdot \vec{v}_2 (\hat{n} \cdot \vec{v}_2)^2 + \frac{6}{5} \vec{S}_1 \times \vec{v}_1 \cdot \vec{v}_2 \hat{n} \cdot \vec{v}_2 + \right.$$

$$\left. 6 \hat{n} \times \vec{S}_1 \cdot \vec{v}_2 \hat{n} \cdot \vec{v}_1 \hat{n} \cdot \vec{v}_2 - \frac{6}{5} \hat{n} \times \vec{S}_1 \cdot \vec{v}_2 \vec{v}_1 \cdot \vec{v}_2 - \frac{38}{35} \hat{n} \times \vec{S}_1 \cdot \vec{v}_2 \vec{v}_2 \cdot \vec{v}_2 \right) m_2^3 \}$$

$$\left\{ \text{DiagSet}[3, 1, 151], \right. , \left. \frac{G^3 m_1^2 m_2 \left( \frac{4}{5} \hat{n} \cdot \vec{v}_1 \vec{S}_1 \times \vec{v}_1 \cdot \vec{v}_2 - \frac{12}{5} \vec{v}_1 \cdot \vec{v}_2 \hat{n} \times \vec{S}_1 \cdot \vec{v}_1 \right)}{r^4} \right\}$$
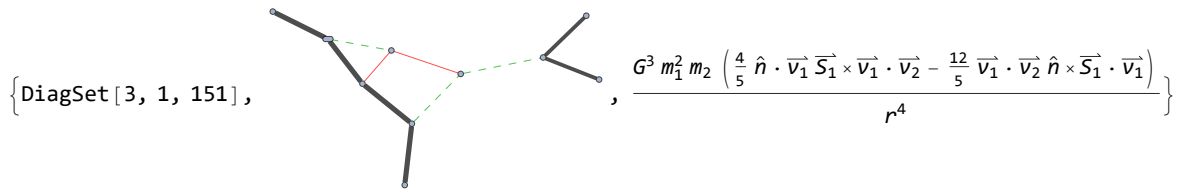

$$\left\{ \text{DiagSet}[3, 1, 152], \right. , \left. \frac{8 G^3 m_1^2 m_2 \vec{v}_1 \cdot \vec{v}_1 \hat{n} \times \vec{S}_1 \cdot \vec{v}_1}{5 r^4} \right\}$$
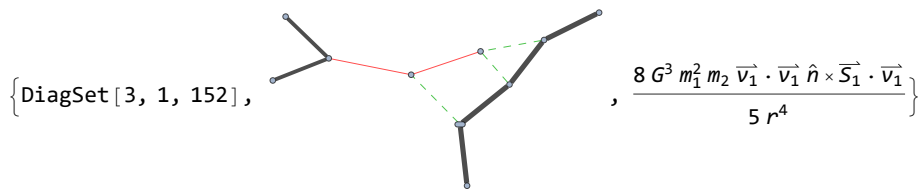

$$\left\{ \text{DiagSet}[3, 1, 153], \right. ,$$
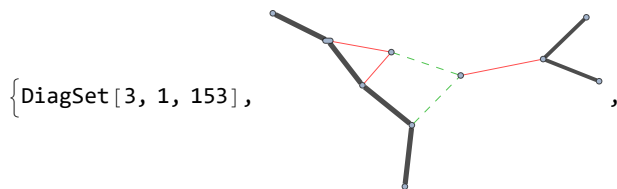

$$\frac{1}{r^3} G^3 m_1^2 m_2 \left( \frac{\frac{4}{5} \hat{n} \cdot \vec{v}_1 \hat{n} \times \vec{S}_1 \cdot \vec{a}_1 + \frac{4}{15} \vec{S}_1 \times \vec{v}_1 \cdot \vec{a}_1 + \frac{4}{5} \hat{n} \cdot \vec{v}_1 \hat{n} \times \vec{S}_1 \cdot \vec{v}_1}{\epsilon_d} - \frac{12}{5} \log\left(\frac{r}{R_\theta}\right) \hat{n} \cdot \vec{v}_1 \hat{n} \times \vec{S}_1 \cdot \vec{a}_1 + \frac{38}{25} \hat{n} \cdot \vec{v}_1 \hat{n} \times \vec{S}_1 \cdot \vec{a}_1 - \right.$$

$$\left. \frac{4}{5} \log\left(\frac{r}{R_\theta}\right) \vec{S}_1 \times \vec{v}_1 \cdot \vec{a}_1 - \frac{34}{25} \vec{S}_1 \times \vec{v}_1 \cdot \vec{a}_1 - \frac{12}{5} \log\left(\frac{r}{R_\theta}\right) \hat{n} \cdot \vec{v}_1 \hat{n} \times \vec{S}_1 \cdot \vec{v}_1 + \frac{38}{25} \hat{n} \cdot \vec{v}_1 \hat{n} \times \vec{S}_1 \cdot \vec{v}_1 \right) +$$

$$\frac{1}{r^4} G^3 m_1^2 m_2 \left( \frac{\frac{16}{35} \vec{v}_1 \cdot \vec{v}_1 \hat{n} \times \vec{S}_1 \cdot \vec{v}_1 - \frac{16}{7} (\hat{n} \cdot \vec{v}_1)^2 \hat{n} \times \vec{S}_1 \cdot \vec{v}_1}{\epsilon_d} + \frac{48}{7} \log\left(\frac{r}{R_\theta}\right) (\hat{n} \cdot \vec{v}_1)^2 \hat{n} \times \vec{S}_1 \cdot \vec{v}_1 - \right.$$

$$\left. \frac{48}{35} \log\left(\frac{r}{R_\theta}\right) \vec{v}_1 \cdot \vec{v}_1 \hat{n} \times \vec{S}_1 \cdot \vec{v}_1 - \frac{288}{49} (\hat{n} \cdot \vec{v}_1)^2 \hat{n} \times \vec{S}_1 \cdot \vec{v}_1 - \frac{2396 \vec{v}_1 \cdot \vec{v}_1 \hat{n} \times \vec{S}_1 \cdot \vec{v}_1}{1225} \right) \}$$

$$\left\{ \text{DiagSet}[3, 1, 154], \right. , \left. \frac{16 G^3 m_2^3 \vec{v}_2 \cdot \vec{v}_2 \hat{n} \times \vec{S}_1 \cdot \vec{v}_2}{5 r^4} \right\}$$
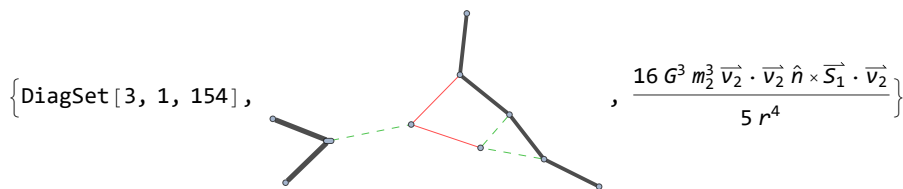

$$\left\{ \text{DiagSet}[3, 1, 155], \right. ,$$
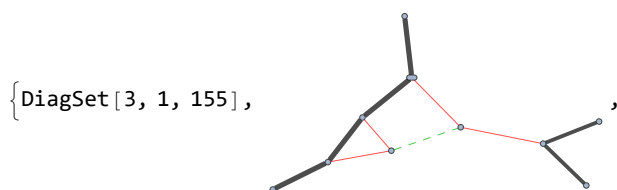

$$\frac{1}{r^3} G^3 m_1^2 m_2 \left( \frac{-\frac{3}{5} \hat{n} \cdot \vec{v}_1 \hat{n} \times \vec{S}_1 \cdot \vec{a}_1 - \frac{1}{5} \vec{S}_1 \times \vec{v}_1 \cdot \vec{a}_1 - \frac{3}{5} \hat{n} \cdot \vec{v}_1 \hat{n} \times \vec{S}_1 \cdot \vec{v}_1}{\epsilon_d} + \frac{9}{5} \log\left(\frac{r}{R_\theta}\right) \hat{n} \cdot \vec{v}_1 \hat{n} \times \vec{S}_1 \cdot \vec{a}_1 - \frac{6}{25} \hat{n} \cdot \vec{v}_1 \hat{n} \times \vec{S}_1 \cdot \vec{a}_1 + \right. \\ \left. \frac{3}{5} \log\left(\frac{r}{R_\theta}\right) \vec{S}_1 \times \vec{v}_1 \cdot \vec{a}_1 - \frac{1}{75} \vec{S}_1 \times \vec{v}_1 \cdot \vec{a}_1 + \frac{9}{5} \log\left(\frac{r}{R_\theta}\right) \hat{n} \cdot \vec{v}_1 \hat{n} \times \vec{S}_1 \cdot \vec{v}_1 - \frac{6}{25} \hat{n} \cdot \vec{v}_1 \hat{n} \times \vec{S}_1 \cdot \vec{v}_1 \right) + \frac{1}{r^4} G^3 m_1^2 m_2 \left( \frac{1}{\epsilon_d} \right. \\ \left( \frac{12}{7} (\hat{n} \cdot \vec{v}_1)^2 \hat{n} \times \vec{S}_1 \cdot \vec{v}_1 - \frac{1}{5} \hat{n} \cdot \vec{v}_1 \vec{S}_1 \times \vec{v}_1 \cdot \vec{v}_2 + \hat{n} \cdot \vec{v}_2 \hat{n} \cdot \vec{v}_1 \hat{n} \times \vec{S}_1 \cdot \vec{v}_1 - \frac{12}{35} \vec{v}_1 \cdot \vec{v}_1 \hat{n} \times \vec{S}_1 \cdot \vec{v}_1 - \frac{1}{5} \vec{v}_1 \cdot \vec{v}_2 \hat{n} \times \vec{S}_1 \cdot \vec{v}_1 \right) - \\ \frac{36}{7} \log\left(\frac{r}{R_\theta}\right) (\hat{n} \cdot \vec{v}_1)^2 \hat{n} \times \vec{S}_1 \cdot \vec{v}_1 + \frac{3}{5} \log\left(\frac{r}{R_\theta}\right) \hat{n} \cdot \vec{v}_1 \vec{S}_1 \times \vec{v}_1 \cdot \vec{v}_2 - 3 \log\left(\frac{r}{R_\theta}\right) \hat{n} \cdot \vec{v}_2 \hat{n} \cdot \vec{v}_1 \hat{n} \times \vec{S}_1 \cdot \vec{v}_1 + \\ \frac{36}{35} \log\left(\frac{r}{R_\theta}\right) \vec{v}_1 \cdot \vec{v}_1 \hat{n} \times \vec{S}_1 \cdot \vec{v}_1 + \frac{3}{5} \log\left(\frac{r}{R_\theta}\right) \vec{v}_1 \cdot \vec{v}_2 \hat{n} \times \vec{S}_1 \cdot \vec{v}_1 + \frac{55}{49} (\hat{n} \cdot \vec{v}_1)^2 \hat{n} \times \vec{S}_1 \cdot \vec{v}_1 + \\ \left. \frac{13}{25} \hat{n} \cdot \vec{v}_1 \vec{S}_1 \times \vec{v}_1 \cdot \vec{v}_2 - 2 \hat{n} \cdot \vec{v}_2 \hat{n} \cdot \vec{v}_1 \hat{n} \times \vec{S}_1 \cdot \vec{v}_1 - \frac{338 \vec{v}_1 \cdot \vec{v}_1 \hat{n} \times \vec{S}_1 \cdot \vec{v}_1}{1225} + \frac{13}{25} \vec{v}_1 \cdot \vec{v}_2 \hat{n} \times \vec{S}_1 \cdot \vec{v}_1 \right) \Big\}$$

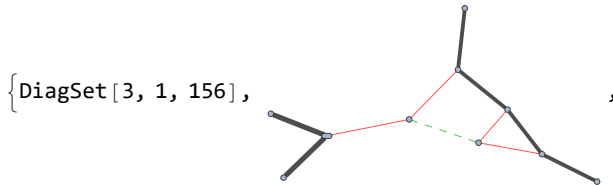

$$\frac{G^3 m_2^3 \left( -2 \hat{n} \cdot \vec{v}_2 \hat{n} \times \vec{a}_1 \cdot \vec{S}_1 + \frac{2}{3} \vec{a}_1 \times \vec{S}_1 \cdot \vec{v}_2 + 2 \hat{n} \cdot \vec{v}_2 \hat{n} \times \vec{S}_1 \cdot \vec{v}_1 - \frac{2}{3} \vec{S}_1 \times \vec{v}_1 \cdot \vec{v}_2 \right)}{r^3} + \frac{1}{r^4} \\ G^3 m_2^3 \left( \frac{3 (\hat{n} \cdot \vec{v}_2)^2 \hat{n} \times \vec{S}_1 \cdot \vec{v}_1 - \frac{6}{5} \hat{n} \cdot \vec{v}_2 \vec{S}_1 \times \vec{v}_1 \cdot \vec{v}_2 - \frac{3}{5} \vec{v}_2 \cdot \vec{v}_2 \hat{n} \times \vec{S}_1 \cdot \vec{v}_1}{\epsilon_d} - 9 \log\left(\frac{r}{R_\theta}\right) (\hat{n} \cdot \vec{v}_2)^2 \hat{n} \times \vec{S}_1 \cdot \vec{v}_1 + \right. \\ \frac{18}{5} \log\left(\frac{r}{R_\theta}\right) \hat{n} \cdot \vec{v}_2 \vec{S}_1 \times \vec{v}_1 \cdot \vec{v}_2 + \frac{9}{5} \log\left(\frac{r}{R_\theta}\right) \vec{v}_2 \cdot \vec{v}_2 \hat{n} \times \vec{S}_1 \cdot \vec{v}_1 + 3 (\hat{n} \cdot \vec{v}_2)^2 \hat{n} \times \vec{S}_1 \cdot \vec{v}_1 - \frac{12}{25} \hat{n} \cdot \vec{v}_2 \vec{S}_1 \times \vec{v}_1 \cdot \vec{v}_2 - \\ \left. 10 \hat{n} \cdot \vec{v}_1 \hat{n} \cdot \vec{v}_2 \hat{n} \times \vec{S}_1 \cdot \vec{v}_1 + 2 \hat{n} \cdot \vec{v}_1 \vec{S}_1 \times \vec{v}_1 \cdot \vec{v}_2 + 2 \vec{v}_1 \cdot \vec{v}_2 \hat{n} \times \vec{S}_1 \cdot \vec{v}_1 - \frac{16}{25} \vec{v}_2 \cdot \vec{v}_2 \hat{n} \times \vec{S}_1 \cdot \vec{v}_1 \right) \Big\}$$

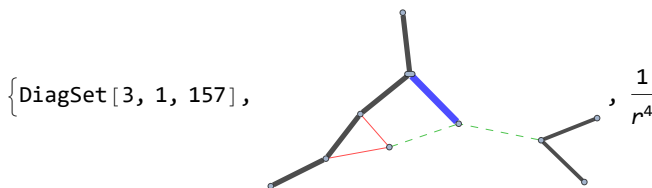

$$G^3 m_1^2 m_2 \left( \frac{1}{\epsilon_d} \left( (\hat{n} \cdot \vec{v}_1)^2 \hat{n} \times \vec{S}_1 \cdot \vec{v}_2 + 2 \hat{n} \cdot \vec{v}_2 \hat{n} \cdot \vec{v}_1 \hat{n} \times \vec{S}_1 \cdot \vec{v}_1 - \frac{1}{5} \vec{v}_1 \cdot \vec{v}_1 \hat{n} \times \vec{S}_1 \cdot \vec{v}_2 - \frac{2}{5} \vec{v}_1 \cdot \vec{v}_2 \hat{n} \times \vec{S}_1 \cdot \vec{v}_1 \right) - \right. \\ 3 \log\left(\frac{r}{R_\theta}\right) (\hat{n} \cdot \vec{v}_1)^2 \hat{n} \times \vec{S}_1 \cdot \vec{v}_2 - 6 \log\left(\frac{r}{R_\theta}\right) \hat{n} \cdot \vec{v}_2 \hat{n} \cdot \vec{v}_1 \hat{n} \times \vec{S}_1 \cdot \vec{v}_1 + \\ \frac{3}{5} \log\left(\frac{r}{R_\theta}\right) \vec{v}_1 \cdot \vec{v}_1 \hat{n} \times \vec{S}_1 \cdot \vec{v}_2 + \frac{6}{5} \log\left(\frac{r}{R_\theta}\right) \vec{v}_1 \cdot \vec{v}_2 \hat{n} \times \vec{S}_1 \cdot \vec{v}_1 + 3 (\hat{n} \cdot \vec{v}_1)^2 \hat{n} \times \vec{S}_1 \cdot \vec{v}_2 - \\ \left. \frac{6}{5} \hat{n} \cdot \vec{v}_1 \vec{S}_1 \times \vec{v}_1 \cdot \vec{v}_2 + 12 \hat{n} \cdot \vec{v}_2 \hat{n} \cdot \vec{v}_1 \hat{n} \times \vec{S}_1 \cdot \vec{v}_1 + \frac{8}{25} \vec{v}_1 \cdot \vec{v}_1 \hat{n} \times \vec{S}_1 \cdot \vec{v}_2 - \frac{84}{25} \vec{v}_1 \cdot \vec{v}_2 \hat{n} \times \vec{S}_1 \cdot \vec{v}_1 \right) \Big\}$$

$\{\text{DiagSet}[3, 1, 158],$ 
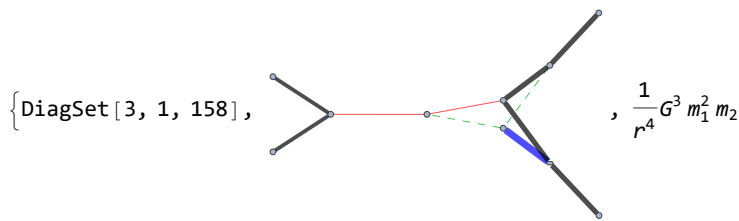
 $, \frac{1}{r^4} G^3 m_1^2 m_2$

$$\left( \frac{1}{\epsilon_d} \left( 3 (\hat{n} \cdot \vec{v}_1)^2 \hat{n} \times \vec{S}_1 \cdot \vec{v}_1 - \frac{3}{5} \hat{n} \cdot \vec{v}_1 \vec{S}_1 \times \vec{v}_1 \cdot \vec{v}_2 + 3 \hat{n} \cdot \vec{v}_2 \hat{n} \cdot \vec{v}_1 \hat{n} \times \vec{S}_1 \cdot \vec{v}_1 - \frac{3}{5} \vec{v}_1 \cdot \vec{v}_1 \hat{n} \times \vec{S}_1 \cdot \vec{v}_1 - \frac{3}{5} \vec{v}_1 \cdot \vec{v}_2 \hat{n} \times \vec{S}_1 \cdot \vec{v}_1 \right) - \right. \\ \left. 9 \log\left(\frac{r}{R_\theta}\right) (\hat{n} \cdot \vec{v}_1)^2 \hat{n} \times \vec{S}_1 \cdot \vec{v}_1 + \frac{9}{5} \log\left(\frac{r}{R_\theta}\right) \hat{n} \cdot \vec{v}_1 \vec{S}_1 \times \vec{v}_1 \cdot \vec{v}_2 - 9 \log\left(\frac{r}{R_\theta}\right) \hat{n} \cdot \vec{v}_2 \hat{n} \cdot \vec{v}_1 \hat{n} \times \vec{S}_1 \cdot \vec{v}_1 + \right. \\ \left. \frac{9}{5} \log\left(\frac{r}{R_\theta}\right) \vec{v}_1 \cdot \vec{v}_1 \hat{n} \times \vec{S}_1 \cdot \vec{v}_1 + \frac{9}{5} \log\left(\frac{r}{R_\theta}\right) \vec{v}_1 \cdot \vec{v}_2 \hat{n} \times \vec{S}_1 \cdot \vec{v}_1 + 5 (\hat{n} \cdot \vec{v}_1)^2 \hat{n} \times \vec{S}_1 \cdot \vec{v}_1 - \right. \\ \left. \frac{16}{25} \hat{n} \cdot \vec{v}_1 \vec{S}_1 \times \vec{v}_1 \cdot \vec{v}_2 + 5 \hat{n} \cdot \vec{v}_2 \hat{n} \cdot \vec{v}_1 \hat{n} \times \vec{S}_1 \cdot \vec{v}_1 - \frac{6}{25} \vec{v}_1 \cdot \vec{v}_1 \hat{n} \times \vec{S}_1 \cdot \vec{v}_1 - \frac{16}{25} \vec{v}_1 \cdot \vec{v}_2 \hat{n} \times \vec{S}_1 \cdot \vec{v}_1 \right) \Big\}$$

$\{\text{DiagSet}[3, 1, 159],$ 
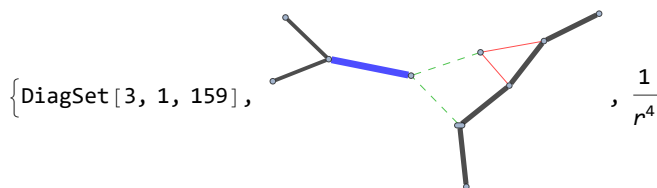
 $, \frac{1}{r^4}$

$$G^3 m_1^2 m_2 \left( \frac{1}{\epsilon_d} \left( -\frac{3}{7} (\hat{n} \cdot \vec{v}_2)^2 \hat{n} \times \vec{S}_1 \cdot \vec{v}_1 + \frac{3}{35} \hat{n} \cdot \vec{v}_2 \vec{S}_1 \times \vec{v}_1 \cdot \vec{v}_2 - \frac{3}{7} \hat{n} \cdot \vec{v}_1 \hat{n} \cdot \vec{v}_2 \hat{n} \times \vec{S}_1 \cdot \vec{v}_2 + \right. \right. \\ \left. \frac{3}{35} \vec{v}_1 \cdot \vec{v}_2 \hat{n} \times \vec{S}_1 \cdot \vec{v}_2 + \frac{3}{35} \vec{v}_2 \cdot \vec{v}_2 \hat{n} \times \vec{S}_1 \cdot \vec{v}_1 \right) + \frac{9}{7} \log\left(\frac{r}{R_\theta}\right) (\hat{n} \cdot \vec{v}_2)^2 \hat{n} \times \vec{S}_1 \cdot \vec{v}_1 - \\ \frac{9}{35} \log\left(\frac{r}{R_\theta}\right) \hat{n} \cdot \vec{v}_2 \vec{S}_1 \times \vec{v}_1 \cdot \vec{v}_2 + \frac{9}{7} \log\left(\frac{r}{R_\theta}\right) \hat{n} \cdot \vec{v}_1 \hat{n} \cdot \vec{v}_2 \hat{n} \times \vec{S}_1 \cdot \vec{v}_2 - \frac{9}{35} \log\left(\frac{r}{R_\theta}\right) \vec{v}_1 \cdot \vec{v}_2 \hat{n} \times \vec{S}_1 \cdot \vec{v}_2 - \\ \frac{9}{35} \log\left(\frac{r}{R_\theta}\right) \vec{v}_2 \cdot \vec{v}_2 \hat{n} \times \vec{S}_1 \cdot \vec{v}_1 - \frac{40}{49} (\hat{n} \cdot \vec{v}_2)^2 \hat{n} \times \vec{S}_1 \cdot \vec{v}_1 + \frac{417 \hat{n} \cdot \vec{v}_2 \vec{S}_1 \times \vec{v}_1 \cdot \vec{v}_2}{1225} - \\ \left. \frac{61}{49} \hat{n} \cdot \vec{v}_1 \hat{n} \cdot \vec{v}_2 \hat{n} \times \vec{S}_1 \cdot \vec{v}_2 - \frac{108 \vec{v}_1 \cdot \vec{v}_2 \hat{n} \times \vec{S}_1 \cdot \vec{v}_2}{1225} + \frac{277 \vec{v}_2 \cdot \vec{v}_2 \hat{n} \times \vec{S}_1 \cdot \vec{v}_1}{1225} \right) \Big\}$$

$\{\text{DiagSet}[3, 1, 160],$ 
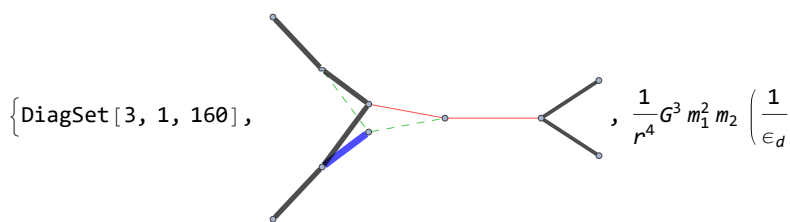
 $, \frac{1}{r^4} G^3 m_1^2 m_2 \left( \frac{1}{\epsilon_d} \right.$

$$\left( -\frac{15}{7} (\hat{n} \cdot \vec{v}_1)^2 \hat{n} \times \vec{S}_1 \cdot \vec{v}_1 - \frac{3}{5} \hat{n} \cdot \vec{v}_1 \vec{S}_1 \times \vec{v}_1 \cdot \vec{v}_2 + 3 \hat{n} \cdot \vec{v}_2 \hat{n} \cdot \vec{v}_1 \hat{n} \times \vec{S}_1 \cdot \vec{v}_1 + \frac{3}{7} \vec{v}_1 \cdot \vec{v}_1 \hat{n} \times \vec{S}_1 \cdot \vec{v}_1 - \frac{3}{5} \vec{v}_1 \cdot \vec{v}_2 \hat{n} \times \vec{S}_1 \cdot \vec{v}_1 \right) + \\ \frac{45}{7} \log\left(\frac{r}{R_\theta}\right) (\hat{n} \cdot \vec{v}_1)^2 \hat{n} \times \vec{S}_1 \cdot \vec{v}_1 + \frac{9}{5} \log\left(\frac{r}{R_\theta}\right) \hat{n} \cdot \vec{v}_1 \vec{S}_1 \times \vec{v}_1 \cdot \vec{v}_2 - 9 \log\left(\frac{r}{R_\theta}\right) \hat{n} \cdot \vec{v}_2 \hat{n} \cdot \vec{v}_1 \hat{n} \times \vec{S}_1 \cdot \vec{v}_1 - \\ \frac{9}{7} \log\left(\frac{r}{R_\theta}\right) \vec{v}_1 \cdot \vec{v}_1 \hat{n} \times \vec{S}_1 \cdot \vec{v}_1 + \frac{9}{5} \log\left(\frac{r}{R_\theta}\right) \vec{v}_1 \cdot \vec{v}_2 \hat{n} \times \vec{S}_1 \cdot \vec{v}_1 - \frac{221}{49} (\hat{n} \cdot \vec{v}_1)^2 \hat{n} \times \vec{S}_1 \cdot \vec{v}_1 - \\ \left. \frac{56}{25} \hat{n} \cdot \vec{v}_1 \vec{S}_1 \times \vec{v}_1 \cdot \vec{v}_2 + 13 \hat{n} \cdot \vec{v}_2 \hat{n} \cdot \vec{v}_1 \hat{n} \times \vec{S}_1 \cdot \vec{v}_1 + \frac{40}{49} \vec{v}_1 \cdot \vec{v}_1 \hat{n} \times \vec{S}_1 \cdot \vec{v}_1 - \frac{56}{25} \vec{v}_1 \cdot \vec{v}_2 \hat{n} \times \vec{S}_1 \cdot \vec{v}_1 \right) \Big\}$$

$\{\text{DiagSet}[3, 1, 161],$  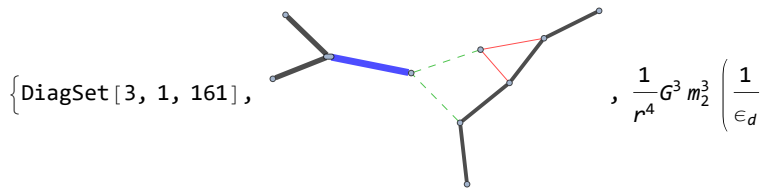 ,  $\frac{1}{r^4} G^3 m_2^3 \left( \frac{1}{\epsilon_d} \right.$

$$\left( \frac{8}{7} (\hat{n} \cdot \vec{v}_2)^2 \hat{n} \times \vec{S}_1 \cdot \vec{v}_1 - \frac{3}{5} \hat{n} \cdot \vec{v}_2 \vec{S}_1 \times \vec{v}_1 \cdot \vec{v}_2 - \frac{5}{7} \hat{n} \cdot \vec{v}_1 \hat{n} \cdot \vec{v}_2 \hat{n} \times \vec{S}_1 \cdot \vec{v}_2 + \frac{1}{7} \vec{v}_1 \cdot \vec{v}_2 \hat{n} \times \vec{S}_1 \cdot \vec{v}_2 - \frac{8}{35} \vec{v}_2 \cdot \vec{v}_2 \hat{n} \times \vec{S}_1 \cdot \vec{v}_1 \right) -$$

$$\frac{24}{7} \log\left(\frac{r}{R_\theta}\right) (\hat{n} \cdot \vec{v}_2)^2 \hat{n} \times \vec{S}_1 \cdot \vec{v}_1 + \frac{9}{5} \log\left(\frac{r}{R_\theta}\right) \hat{n} \cdot \vec{v}_2 \vec{S}_1 \times \vec{v}_1 \cdot \vec{v}_2 + \frac{15}{7} \log\left(\frac{r}{R_\theta}\right) \hat{n} \cdot \vec{v}_1 \hat{n} \cdot \vec{v}_2 \hat{n} \times \vec{S}_1 \cdot \vec{v}_2 -$$

$$\frac{3}{7} \log\left(\frac{r}{R_\theta}\right) \vec{v}_1 \cdot \vec{v}_2 \hat{n} \times \vec{S}_1 \cdot \vec{v}_2 + \frac{24}{35} \log\left(\frac{r}{R_\theta}\right) \vec{v}_2 \cdot \vec{v}_2 \hat{n} \times \vec{S}_1 \cdot \vec{v}_1 + \frac{32}{49} (\hat{n} \cdot \vec{v}_2)^2 \hat{n} \times \vec{S}_1 \cdot \vec{v}_1 -$$

$$\frac{6}{25} \hat{n} \cdot \vec{v}_2 \vec{S}_1 \times \vec{v}_1 \cdot \vec{v}_2 - \frac{83}{49} \hat{n} \cdot \vec{v}_1 \hat{n} \cdot \vec{v}_2 \hat{n} \times \vec{S}_1 \cdot \vec{v}_2 - \frac{122}{49} \vec{v}_1 \cdot \vec{v}_2 \hat{n} \times \vec{S}_1 \cdot \vec{v}_2 + \frac{2248 \vec{v}_2 \cdot \vec{v}_2 \hat{n} \times \vec{S}_1 \cdot \vec{v}_1}{1225} \Bigg\}$$

$\{\text{DiagSet}[3, 1, 162],$  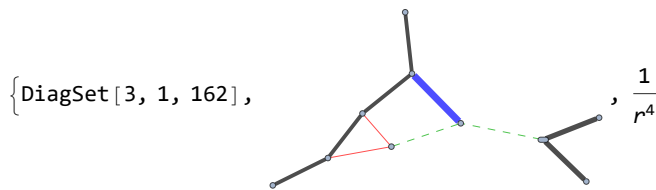 ,  $\frac{1}{r^4}$

$$G^3 m_2^3 \left( \frac{10 (\hat{n} \cdot \vec{v}_2)^2 \hat{n} \times \vec{S}_1 \cdot \vec{v}_2 - 2 \vec{v}_2 \cdot \vec{v}_2 \hat{n} \times \vec{S}_1 \cdot \vec{v}_2}{\epsilon_d} - 30 \log\left(\frac{r}{R_\theta}\right) (\hat{n} \cdot \vec{v}_2)^2 \hat{n} \times \vec{S}_1 \cdot \vec{v}_2 + \right.$$

$$\left. 6 \log\left(\frac{r}{R_\theta}\right) \vec{v}_2 \cdot \vec{v}_2 \hat{n} \times \vec{S}_1 \cdot \vec{v}_2 + 21 (\hat{n} \cdot \vec{v}_2)^2 \hat{n} \times \vec{S}_1 \cdot \vec{v}_2 - 3 \vec{v}_2 \cdot \vec{v}_2 \hat{n} \times \vec{S}_1 \cdot \vec{v}_2 \right\}$$

$\{\text{DiagSet}[3, 1, 163],$  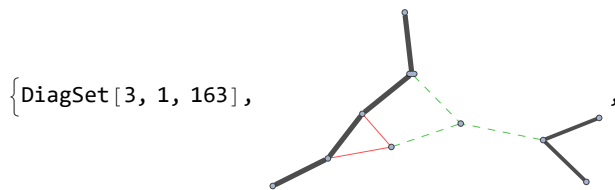 ,

$$\frac{1}{r^3} m_1^2 m_2 \left( -\frac{4}{5} \log\left(\frac{r}{R_\theta}\right) \vec{S}_1 \times \vec{v}_1 \cdot \vec{v}_2 - \frac{2}{75} \vec{S}_1 \times \vec{v}_1 \cdot \vec{v}_2 + \frac{28}{75} \vec{S}_1 \times \vec{a}_1 \cdot \vec{v}_2 - \frac{2}{75} \vec{S}_1 \times \vec{v}_1 \cdot \vec{a}_2 + \frac{34}{25} \hat{n} \times \vec{S}_1 \cdot \vec{v}_2 \hat{n} \cdot \vec{a}_1 - \right.$$

$$\frac{17}{25} \hat{n} \times \vec{S}_1 \cdot \vec{v}_1 \hat{n} \cdot \vec{a}_2 - \frac{11}{25} \hat{n} \times \vec{S}_1 \cdot \vec{v}_2 \hat{n} \cdot \vec{v}_1 - \frac{4}{25} \hat{n} \times \vec{S}_1 \cdot \vec{a}_2 \hat{n} \cdot \vec{v}_1 - \frac{24}{25} \hat{n} \times \vec{S}_1 \cdot \vec{v}_1 \hat{n} \cdot \vec{v}_2 - \frac{9}{25} \hat{n} \times \vec{S}_1 \cdot \vec{a}_1 \hat{n} \cdot \vec{v}_2 -$$

$$\frac{4}{5} \vec{S}_1 \times \vec{a}_1 \cdot \vec{v}_2 \log\left(\frac{r}{R_\theta}\right) + \frac{1}{5} \vec{S}_1 \times \vec{v}_1 \cdot \vec{a}_2 \log\left(\frac{r}{R_\theta}\right) - \frac{6}{5} \hat{n} \times \vec{S}_1 \cdot \vec{v}_2 \hat{n} \cdot \vec{a}_1 \log\left(\frac{r}{R_\theta}\right) + \frac{3}{5} \hat{n} \times \vec{S}_1 \cdot \vec{v}_1 \hat{n} \cdot \vec{a}_2 \log\left(\frac{r}{R_\theta}\right) -$$

$$\frac{6}{5} \hat{n} \times \vec{S}_1 \cdot \vec{v}_2 \hat{n} \cdot \vec{v}_1 \log\left(\frac{r}{R_\theta}\right) + \frac{6}{5} \hat{n} \times \vec{S}_1 \cdot \vec{a}_2 \hat{n} \cdot \vec{v}_1 \log\left(\frac{r}{R_\theta}\right) + \frac{6}{5} \hat{n} \times \vec{S}_1 \cdot \vec{v}_1 \hat{n} \cdot \vec{v}_2 \log\left(\frac{r}{R_\theta}\right) +$$

$$\frac{6}{5} \hat{n} \times \vec{S}_1 \cdot \vec{a}_1 \hat{n} \cdot \vec{v}_2 \log\left(\frac{r}{R_\theta}\right) + \frac{1}{\epsilon_d} \left( \frac{4}{15} \vec{S}_1 \times \vec{v}_1 \cdot \vec{v}_2 + \frac{4}{15} \vec{S}_1 \times \vec{a}_1 \cdot \vec{v}_2 - \frac{1}{15} \vec{S}_1 \times \vec{v}_1 \cdot \vec{a}_2 + \frac{2}{5} \hat{n} \times \vec{S}_1 \cdot \vec{v}_2 \hat{n} \cdot \vec{a}_1 - \right.$$

$$\left. \frac{1}{5} \hat{n} \times \vec{S}_1 \cdot \vec{v}_1 \hat{n} \cdot \vec{a}_2 + \frac{2}{5} \hat{n} \times \vec{S}_1 \cdot \vec{v}_2 \hat{n} \cdot \vec{v}_1 - \frac{2}{5} \hat{n} \times \vec{S}_1 \cdot \vec{a}_2 \hat{n} \cdot \vec{v}_1 - \frac{2}{5} \hat{n} \times \vec{S}_1 \cdot \vec{v}_1 \hat{n} \cdot \vec{v}_2 - \frac{2}{5} \hat{n} \times \vec{S}_1 \cdot \vec{a}_1 \hat{n} \cdot \vec{v}_2 \right) \Bigg) G^3 +$$

$$\frac{1}{r^4} m_1^2 m_2 \left( -\frac{201}{49} \hat{n} \times \vec{S}_1 \cdot \vec{v}_2 (\hat{n} \cdot \vec{v}_1)^2 + \frac{51}{7} \hat{n} \times \vec{S}_1 \cdot \vec{v}_2 \log\left(\frac{r}{R_\theta}\right) (\hat{n} \cdot \vec{v}_1)^2 - \frac{1573 \vec{S}_1 \times \vec{v}_1 \cdot \vec{v}_2 \hat{n} \cdot \vec{v}_1}{1225} - \right.$$

$$\frac{16}{49} \hat{n} \times \vec{S}_1 \cdot \vec{v}_1 \hat{n} \cdot \vec{v}_2 \hat{n} \cdot \vec{v}_1 - 2 \hat{n} \times \vec{S}_1 \cdot \vec{v}_2 \hat{n} \cdot \vec{v}_2 \hat{n} \cdot \vec{v}_1 + \frac{111}{35} \vec{S}_1 \times \vec{v}_1 \cdot \vec{v}_2 \log\left(\frac{r}{R_\theta}\right) \hat{n} \cdot \vec{v}_1 -$$

$$\frac{9}{7} \hat{n} \times \vec{S}_1 \cdot \vec{v}_1 \hat{n} \cdot \vec{v}_2 \log\left(\frac{r}{R_\theta}\right) \hat{n} \cdot \vec{v}_1 + 6 \hat{n} \times \vec{S}_1 \cdot \vec{v}_2 \hat{n} \cdot \vec{v}_2 \log\left(\frac{r}{R_\theta}\right) \hat{n} \cdot \vec{v}_1 - 4 \hat{n} \times \vec{S}_1 \cdot \vec{v}_1 (\hat{n} \cdot \vec{v}_2)^2 +$$

$$\begin{aligned} & \frac{2}{5} \vec{S}_1 \times \vec{v}_1 \cdot \vec{v}_2 \hat{n} \cdot \vec{v}_2 + \frac{1278 \hat{n} \times \vec{S}_1 \cdot \vec{v}_2 \vec{v}_1 \cdot \vec{v}_1}{1225} + \frac{1228 \hat{n} \times \vec{S}_1 \cdot \vec{v}_1 \vec{v}_1 \cdot \vec{v}_2}{1225} + \frac{4}{25} \hat{n} \times \vec{S}_1 \cdot \vec{v}_2 \vec{v}_1 \cdot \vec{v}_2 + \\ & \frac{17}{25} \hat{n} \times \vec{S}_1 \cdot \vec{v}_1 \vec{v}_2 \cdot \vec{v}_2 + 3 \hat{n} \times \vec{S}_1 \cdot \vec{v}_1 (\hat{n} \cdot \vec{v}_2)^2 \log\left(\frac{r}{R_0}\right) - \frac{51}{35} \hat{n} \times \vec{S}_1 \cdot \vec{v}_2 \vec{v}_1 \cdot \vec{v}_1 \log\left(\frac{r}{R_0}\right) + \\ & \frac{9}{35} \hat{n} \times \vec{S}_1 \cdot \vec{v}_1 \vec{v}_1 \cdot \vec{v}_2 \log\left(\frac{r}{R_0}\right) - \frac{6}{5} \hat{n} \times \vec{S}_1 \cdot \vec{v}_2 \vec{v}_1 \cdot \vec{v}_2 \log\left(\frac{r}{R_0}\right) - \frac{3}{5} \hat{n} \times \vec{S}_1 \cdot \vec{v}_1 \vec{v}_2 \cdot \vec{v}_2 \log\left(\frac{r}{R_0}\right) + \frac{1}{\epsilon_d} \\ & \left( -\frac{17}{7} \hat{n} \times \vec{S}_1 \cdot \vec{v}_2 (\hat{n} \cdot \vec{v}_1)^2 - \frac{37}{35} \vec{S}_1 \times \vec{v}_1 \cdot \vec{v}_2 \hat{n} \cdot \vec{v}_1 + \frac{3}{7} \hat{n} \times \vec{S}_1 \cdot \vec{v}_1 \hat{n} \cdot \vec{v}_2 \hat{n} \cdot \vec{v}_1 - 2 \hat{n} \times \vec{S}_1 \cdot \vec{v}_2 \hat{n} \cdot \vec{v}_2 \hat{n} \cdot \vec{v}_1 - \right. \\ & \left. \hat{n} \times \vec{S}_1 \cdot \vec{v}_1 (\hat{n} \cdot \vec{v}_2)^2 + \frac{17}{35} \hat{n} \times \vec{S}_1 \cdot \vec{v}_2 \vec{v}_1 \cdot \vec{v}_1 - \frac{3}{35} \hat{n} \times \vec{S}_1 \cdot \vec{v}_1 \vec{v}_1 \cdot \vec{v}_2 + \frac{2}{5} \hat{n} \times \vec{S}_1 \cdot \vec{v}_2 \vec{v}_1 \cdot \vec{v}_2 + \frac{1}{5} \hat{n} \times \vec{S}_1 \cdot \vec{v}_1 \vec{v}_2 \cdot \vec{v}_2 \right) \Bigg) G^3 \Bigg\} \end{aligned}$$

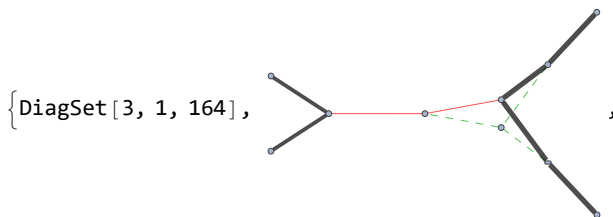

$$\begin{aligned} & \frac{1}{r^3} m_1^2 m_2 \left( 2 \log\left(\frac{r}{R_0}\right) \vec{S}_1 \times \vec{v}_1 \cdot \vec{v}_2 - \frac{1}{3} \vec{S}_1 \times \vec{v}_1 \cdot \vec{v}_2 + \frac{5}{3} \vec{S}_1 \times \vec{a}_1 \cdot \vec{v}_2 + \frac{16}{25} \vec{S}_1 \times \vec{v}_1 \cdot \vec{a}_1 + \frac{2}{3} \vec{S}_1 \times \vec{v}_1 \cdot \vec{a}_2 - \right. \\ & \frac{34}{25} \hat{n} \times \vec{S}_1 \cdot \vec{v}_1 \hat{n} \cdot \vec{a}_1 - 3 \hat{n} \times \vec{S}_1 \cdot \vec{v}_1 \hat{n} \cdot \vec{a}_2 + \frac{3}{5} \hat{n} \times \vec{S}_1 \cdot \vec{v}_1 \hat{n} \cdot \vec{v}_1 + \frac{4}{25} \hat{n} \times \vec{S}_1 \cdot \vec{a}_1 \hat{n} \cdot \vec{v}_1 + 3 \hat{n} \times \vec{S}_1 \cdot \vec{v}_1 \hat{n} \cdot \vec{v}_2 - \\ & 7 \hat{n} \times \vec{S}_1 \cdot \vec{a}_1 \hat{n} \cdot \vec{v}_2 - 2 \vec{S}_1 \times \vec{a}_1 \cdot \vec{v}_2 \log\left(\frac{r}{R_0}\right) - \frac{4}{5} \vec{S}_1 \times \vec{v}_1 \cdot \vec{a}_1 \log\left(\frac{r}{R_0}\right) - \vec{S}_1 \times \vec{v}_1 \cdot \vec{a}_2 \log\left(\frac{r}{R_0}\right) + \\ & \frac{6}{5} \hat{n} \times \vec{S}_1 \cdot \vec{v}_1 \hat{n} \cdot \vec{a}_1 \log\left(\frac{r}{R_0}\right) + 3 \hat{n} \times \vec{S}_1 \cdot \vec{v}_1 \hat{n} \cdot \vec{a}_2 \log\left(\frac{r}{R_0}\right) - 3 \hat{n} \times \vec{S}_1 \cdot \vec{v}_1 \hat{n} \cdot \vec{v}_1 \log\left(\frac{r}{R_0}\right) - \\ & \frac{6}{5} \hat{n} \times \vec{S}_1 \cdot \vec{a}_1 \hat{n} \cdot \vec{v}_1 \log\left(\frac{r}{R_0}\right) - 6 \hat{n} \times \vec{S}_1 \cdot \vec{v}_1 \hat{n} \cdot \vec{v}_2 \log\left(\frac{r}{R_0}\right) + 6 \hat{n} \times \vec{S}_1 \cdot \vec{a}_1 \hat{n} \cdot \vec{v}_2 \log\left(\frac{r}{R_0}\right) + \frac{1}{\epsilon_d} \\ & \left( -\frac{2}{3} \vec{S}_1 \times \vec{v}_1 \cdot \vec{v}_2 + \frac{2}{3} \vec{S}_1 \times \vec{a}_1 \cdot \vec{v}_2 + \frac{4}{15} \vec{S}_1 \times \vec{v}_1 \cdot \vec{a}_1 + \frac{1}{3} \vec{S}_1 \times \vec{v}_1 \cdot \vec{a}_2 - \frac{2}{5} \hat{n} \times \vec{S}_1 \cdot \vec{v}_1 \hat{n} \cdot \vec{a}_1 - \hat{n} \times \vec{S}_1 \cdot \vec{v}_1 \hat{n} \cdot \vec{a}_2 + \right. \\ & \left. \hat{n} \times \vec{S}_1 \cdot \vec{v}_1 \hat{n} \cdot \vec{v}_1 + \frac{2}{5} \hat{n} \times \vec{S}_1 \cdot \vec{a}_1 \hat{n} \cdot \vec{v}_1 + 2 \hat{n} \times \vec{S}_1 \cdot \vec{v}_1 \hat{n} \cdot \vec{v}_2 - 2 \hat{n} \times \vec{S}_1 \cdot \vec{a}_1 \hat{n} \cdot \vec{v}_2 \right) \Bigg) G^3 + \frac{1}{r^4} \\ & m_1^2 m_2 \left( -\frac{48}{7} \hat{n} \times \vec{S}_1 \cdot \vec{v}_1 (\hat{n} \cdot \vec{v}_1)^2 + 9 \hat{n} \times \vec{S}_1 \cdot \vec{v}_1 \log\left(\frac{r}{R_0}\right) (\hat{n} \cdot \vec{v}_1)^2 + \frac{38}{25} \vec{S}_1 \times \vec{v}_1 \cdot \vec{v}_2 \hat{n} \cdot \vec{v}_1 - 10 \hat{n} \times \vec{S}_1 \cdot \vec{v}_1 \hat{n} \cdot \vec{v}_2 \hat{n} \cdot \vec{v}_1 - \right. \\ & \frac{12}{5} \vec{S}_1 \times \vec{v}_1 \cdot \vec{v}_2 \log\left(\frac{r}{R_0}\right) \hat{n} \cdot \vec{v}_1 + 12 \hat{n} \times \vec{S}_1 \cdot \vec{v}_1 \hat{n} \cdot \vec{v}_2 \log\left(\frac{r}{R_0}\right) \hat{n} \cdot \vec{v}_1 - 18 \hat{n} \times \vec{S}_1 \cdot \vec{v}_1 (\hat{n} \cdot \vec{v}_2)^2 + 6 \vec{S}_1 \times \vec{v}_1 \cdot \vec{v}_2 \hat{n} \cdot \vec{v}_2 + \\ & \frac{2}{175} \hat{n} \times \vec{S}_1 \cdot \vec{v}_1 \vec{v}_1 \cdot \vec{v}_1 + \frac{38}{25} \hat{n} \times \vec{S}_1 \cdot \vec{v}_1 \vec{v}_1 \cdot \vec{v}_2 + 3 \hat{n} \times \vec{S}_1 \cdot \vec{v}_1 \vec{v}_2 \cdot \vec{v}_2 + 15 \hat{n} \times \vec{S}_1 \cdot \vec{v}_1 (\hat{n} \cdot \vec{v}_2)^2 \log\left(\frac{r}{R_0}\right) - \\ & 6 \vec{S}_1 \times \vec{v}_1 \cdot \vec{v}_2 \hat{n} \cdot \vec{v}_2 \log\left(\frac{r}{R_0}\right) - \frac{9}{5} \hat{n} \times \vec{S}_1 \cdot \vec{v}_1 \vec{v}_1 \cdot \vec{v}_1 \log\left(\frac{r}{R_0}\right) - \frac{12}{5} \hat{n} \times \vec{S}_1 \cdot \vec{v}_1 \vec{v}_1 \cdot \vec{v}_2 \log\left(\frac{r}{R_0}\right) - \\ & 3 \hat{n} \times \vec{S}_1 \cdot \vec{v}_1 \vec{v}_2 \cdot \vec{v}_2 \log\left(\frac{r}{R_0}\right) + \frac{1}{\epsilon_d} \left( -3 \hat{n} \times \vec{S}_1 \cdot \vec{v}_1 (\hat{n} \cdot \vec{v}_1)^2 + \frac{4}{5} \vec{S}_1 \times \vec{v}_1 \cdot \vec{v}_2 \hat{n} \cdot \vec{v}_1 - 4 \hat{n} \times \vec{S}_1 \cdot \vec{v}_1 \hat{n} \cdot \vec{v}_2 \hat{n} \cdot \vec{v}_1 - \right. \\ & \left. 5 \hat{n} \times \vec{S}_1 \cdot \vec{v}_1 (\hat{n} \cdot \vec{v}_2)^2 + 2 \vec{S}_1 \times \vec{v}_1 \cdot \vec{v}_2 \hat{n} \cdot \vec{v}_2 + \frac{3}{5} \hat{n} \times \vec{S}_1 \cdot \vec{v}_1 \vec{v}_1 \cdot \vec{v}_1 + \frac{4}{5} \hat{n} \times \vec{S}_1 \cdot \vec{v}_1 \vec{v}_1 \cdot \vec{v}_2 + \hat{n} \times \vec{S}_1 \cdot \vec{v}_1 \vec{v}_2 \cdot \vec{v}_2 \right) \Bigg) G^3 \Bigg\} \end{aligned}$$

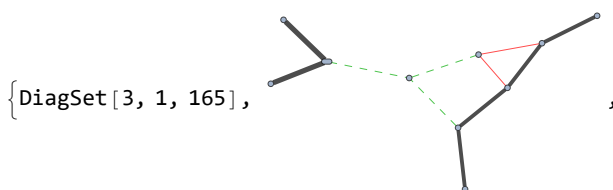

$$\frac{1}{r^3} G^3 m_2^3 \left( \frac{4 \hat{n} \cdot \vec{v}_2 \hat{n} \times \vec{a}_2 \cdot \vec{S}_1 - \frac{4}{3} \vec{a}_2 \times \vec{S}_1 \cdot \vec{v}_2 + \frac{7}{5} \hat{n} \cdot \vec{v}_2 \hat{n} \times \vec{S}_1 \cdot \vec{v}_2}{\epsilon_d} - 12 \log \left( \frac{r}{R_\theta} \right) \hat{n} \cdot \vec{v}_2 \hat{n} \times \vec{a}_2 \cdot \vec{S}_1 + \right. \\ \left. 4 \hat{n} \cdot \vec{v}_2 \hat{n} \times \vec{a}_2 \cdot \vec{S}_1 + 4 \log \left( \frac{r}{R_\theta} \right) \vec{a}_2 \times \vec{S}_1 \cdot \vec{v}_2 - \frac{21}{5} \log \left( \frac{r}{R_\theta} \right) \hat{n} \cdot \vec{v}_2 \hat{n} \times \vec{S}_1 \cdot \vec{v}_2 + \frac{9}{25} \hat{n} \cdot \vec{v}_2 \hat{n} \times \vec{S}_1 \cdot \vec{v}_2 \right) + \frac{1}{r^4} \\ G^3 m_2^3 \left( \frac{1}{\epsilon_d} \left( -\frac{80}{7} (\hat{n} \cdot \vec{v}_2)^2 \hat{n} \times \vec{S}_1 \cdot \vec{v}_2 - \frac{7}{5} \hat{n} \cdot \vec{v}_2 \vec{S}_1 \times \vec{v}_1 \cdot \vec{v}_2 - 7 \hat{n} \cdot \vec{v}_1 \hat{n} \cdot \vec{v}_2 \hat{n} \times \vec{S}_1 \cdot \vec{v}_2 + \frac{7}{5} \vec{v}_1 \cdot \vec{v}_2 \hat{n} \times \vec{S}_1 \cdot \vec{v}_2 + \right. \right. \\ \left. \frac{16}{7} \vec{v}_2 \cdot \vec{v}_2 \hat{n} \times \vec{S}_1 \cdot \vec{v}_2 \right) + \frac{240}{7} \log \left( \frac{r}{R_\theta} \right) (\hat{n} \cdot \vec{v}_2)^2 \hat{n} \times \vec{S}_1 \cdot \vec{v}_2 + \frac{21}{5} \log \left( \frac{r}{R_\theta} \right) \hat{n} \cdot \vec{v}_2 \vec{S}_1 \times \vec{v}_1 \cdot \vec{v}_2 + 21 \log \left( \frac{r}{R_\theta} \right) \hat{n} \cdot \vec{v}_1 \\ \hat{n} \cdot \vec{v}_2 \hat{n} \times \vec{S}_1 \cdot \vec{v}_2 - \frac{21}{5} \log \left( \frac{r}{R_\theta} \right) \vec{v}_1 \cdot \vec{v}_2 \hat{n} \times \vec{S}_1 \cdot \vec{v}_2 - \frac{48}{7} \log \left( \frac{r}{R_\theta} \right) \vec{v}_2 \cdot \vec{v}_2 \hat{n} \times \vec{S}_1 \cdot \vec{v}_2 - \frac{1223}{49} (\hat{n} \cdot \vec{v}_2)^2 \hat{n} \times \vec{S}_1 \cdot \vec{v}_2 - \\ \left. \frac{9}{25} \hat{n} \cdot \vec{v}_2 \vec{S}_1 \times \vec{v}_1 \cdot \vec{v}_2 - 6 \hat{n} \cdot \vec{v}_1 \hat{n} \cdot \vec{v}_2 \hat{n} \times \vec{S}_1 \cdot \vec{v}_2 + \frac{9}{25} \vec{v}_1 \cdot \vec{v}_2 \hat{n} \times \vec{S}_1 \cdot \vec{v}_2 + \frac{1209}{245} \vec{v}_2 \cdot \vec{v}_2 \hat{n} \times \vec{S}_1 \cdot \vec{v}_2 \right) \Big\}$$

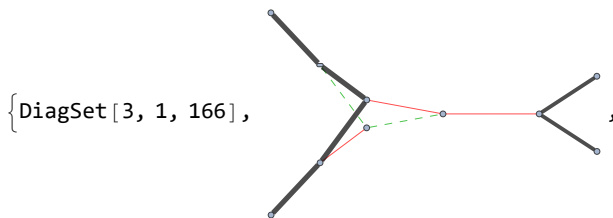

$$\frac{1}{r^3} m_1^2 m_2 \left( 4 \log \left( \frac{r}{R_\theta} \right) \frac{1}{\vec{S}_1 \times \vec{v}_1 \cdot \vec{v}_2} - \frac{2}{3} \frac{1}{\vec{S}_1 \times \vec{v}_1 \cdot \vec{v}_2} - \frac{2}{3} \vec{S}_1 \times \vec{a}_1 \cdot \vec{v}_2 + \frac{2}{3} \vec{S}_1 \times \vec{v}_1 \cdot \vec{a}_1 + \right. \\ \left. 6 \hat{n} \times \vec{S}_1 \cdot \vec{v}_1 \hat{n} \cdot \vec{v}_1 + 6 \hat{n} \times \vec{S}_1 \cdot \vec{a}_1 \hat{n} \cdot \vec{v}_1 + 6 \hat{n} \times \vec{S}_1 \cdot \vec{v}_1 \hat{n} \cdot \vec{v}_2 + 6 \hat{n} \times \vec{S}_1 \cdot \vec{a}_1 \hat{n} \cdot \vec{v}_2 + 4 \vec{S}_1 \times \vec{a}_1 \cdot \vec{v}_2 \log \left( \frac{r}{R_\theta} \right) - \right. \\ \left. 4 \vec{S}_1 \times \vec{v}_1 \cdot \vec{a}_1 \log \left( \frac{r}{R_\theta} \right) - 12 \hat{n} \times \vec{S}_1 \cdot \vec{v}_1 \hat{n} \cdot \vec{v}_1 \log \left( \frac{r}{R_\theta} \right) - 12 \hat{n} \times \vec{S}_1 \cdot \vec{a}_1 \hat{n} \cdot \vec{v}_1 \log \left( \frac{r}{R_\theta} \right) - \right. \\ \left. 12 \hat{n} \times \vec{S}_1 \cdot \vec{v}_1 \hat{n} \cdot \vec{v}_2 \log \left( \frac{r}{R_\theta} \right) - 12 \hat{n} \times \vec{S}_1 \cdot \vec{a}_1 \hat{n} \cdot \vec{v}_2 \log \left( \frac{r}{R_\theta} \right) + \frac{1}{\epsilon_d} \left( -\frac{4}{3} \frac{1}{\vec{S}_1 \times \vec{v}_1 \cdot \vec{v}_2} - \frac{4}{3} \vec{S}_1 \times \vec{a}_1 \cdot \vec{v}_2 + \right. \right. \\ \left. \frac{4}{3} \vec{S}_1 \times \vec{v}_1 \cdot \vec{a}_1 + 4 \hat{n} \times \vec{S}_1 \cdot \vec{v}_1 \hat{n} \cdot \vec{v}_1 + 4 \hat{n} \times \vec{S}_1 \cdot \vec{a}_1 \hat{n} \cdot \vec{v}_1 + 4 \hat{n} \times \vec{S}_1 \cdot \vec{v}_1 \hat{n} \cdot \vec{v}_2 + 4 \hat{n} \times \vec{S}_1 \cdot \vec{a}_1 \hat{n} \cdot \vec{v}_2 \right) \Big) G^3 + \frac{1}{r^4} \\ m_1^2 m_2 \left( -14 \hat{n} \times \vec{S}_1 \cdot \vec{v}_1 (\hat{n} \cdot \vec{v}_1)^2 + 18 \hat{n} \times \vec{S}_1 \cdot \vec{v}_1 \log \left( \frac{r}{R_\theta} \right) (\hat{n} \cdot \vec{v}_1)^2 + \frac{52}{25} \vec{S}_1 \times \vec{v}_1 \cdot \vec{v}_2 \hat{n} \cdot \vec{v}_1 - 14 \hat{n} \times \vec{S}_1 \cdot \vec{v}_1 \hat{n} \cdot \vec{v}_2 \hat{n} \cdot \vec{v}_1 - \right. \\ \frac{18}{5} \vec{S}_1 \times \vec{v}_1 \cdot \vec{v}_2 \log \left( \frac{r}{R_\theta} \right) \hat{n} \cdot \vec{v}_1 + 18 \hat{n} \times \vec{S}_1 \cdot \vec{v}_1 \hat{n} \cdot \vec{v}_2 \log \left( \frac{r}{R_\theta} \right) \hat{n} \cdot \vec{v}_1 + \frac{109}{50} \hat{n} \times \vec{S}_1 \cdot \vec{v}_1 \vec{v}_1 \cdot \vec{v}_1 + \frac{52}{25} \hat{n} \times \vec{S}_1 \cdot \vec{v}_1 \vec{v}_1 \cdot \vec{v}_2 + \\ \frac{3}{10} \hat{n} \times \vec{S}_1 \cdot \vec{v}_1 \vec{v}_2 \cdot \vec{v}_2 - \frac{18}{5} \hat{n} \times \vec{S}_1 \cdot \vec{v}_1 \vec{v}_1 \cdot \vec{v}_1 \log \left( \frac{r}{R_\theta} \right) - \frac{18}{5} \hat{n} \times \vec{S}_1 \cdot \vec{v}_1 \vec{v}_1 \cdot \vec{v}_2 \log \left( \frac{r}{R_\theta} \right) + \frac{1}{\epsilon_d} \left( -6 \hat{n} \times \vec{S}_1 \cdot \vec{v}_1 (\hat{n} \cdot \vec{v}_1)^2 + \right. \\ \left. \frac{6}{5} \vec{S}_1 \times \vec{v}_1 \cdot \vec{v}_2 \hat{n} \cdot \vec{v}_1 - 6 \hat{n} \times \vec{S}_1 \cdot \vec{v}_1 \hat{n} \cdot \vec{v}_2 \hat{n} \cdot \vec{v}_1 + \frac{6}{5} \hat{n} \times \vec{S}_1 \cdot \vec{v}_1 \vec{v}_1 \cdot \vec{v}_1 + \frac{6}{5} \hat{n} \times \vec{S}_1 \cdot \vec{v}_1 \vec{v}_1 \cdot \vec{v}_2 \right) \Big) G^3 \Big\}$$

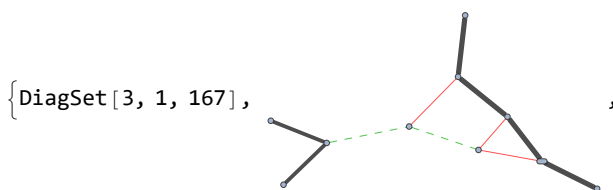

$$\frac{1}{r^3} G^3 m_1^2 m_2 \left( \frac{-4 \hat{n} \cdot \vec{v}_2 \hat{n} \times \vec{S}_1 \cdot \vec{a}_1 + \frac{4}{3} \vec{S}_1 \times \vec{a}_1 \cdot \vec{v}_2 - 4 \hat{n} \cdot \vec{v}_2 \hat{n} \times \vec{S}_1 \cdot \vec{v}_1 + \frac{4}{3} \frac{1}{\vec{S}_1 \times \vec{v}_1 \cdot \vec{v}_2}}{\epsilon_d} + \right.$$

$$\begin{aligned}
& 12 \log\left(\frac{r}{R_\theta}\right) \hat{n} \cdot \vec{v}_2 \hat{n} \times \vec{S}_1 \cdot \vec{a}_1 - 6 \hat{n} \cdot \vec{v}_2 \hat{n} \times \vec{S}_1 \cdot \vec{a}_1 - 4 \log\left(\frac{r}{R_\theta}\right) \vec{S}_1 \times \vec{a}_1 \cdot \vec{v}_2 - 2 \vec{S}_1 \times \vec{a}_1 \cdot \vec{v}_2 + \\
& 12 \log\left(\frac{r}{R_\theta}\right) \hat{n} \cdot \vec{v}_2 \hat{n} \times \vec{S}_1 \cdot \vec{v}_1 - 6 \hat{n} \cdot \vec{v}_2 \hat{n} \times \vec{S}_1 \cdot \vec{v}_1 - 4 \log\left(\frac{r}{R_\theta}\right) \vec{S}_1 \times \vec{v}_1 \cdot \vec{v}_2 - 2 \vec{S}_1 \times \vec{v}_1 \cdot \vec{v}_2 \Bigg) + \\
& \frac{1}{r^4} G^3 m_1^2 m_2 \left( \frac{-\frac{16}{5} \hat{n} \cdot \vec{v}_1 \vec{S}_1 \times \vec{v}_1 \cdot \vec{v}_2 + 16 \hat{n} \cdot \vec{v}_2 \hat{n} \cdot \vec{v}_1 \hat{n} \times \vec{S}_1 \cdot \vec{v}_1 - \frac{16}{5} \vec{v}_1 \cdot \vec{v}_2 \hat{n} \times \vec{S}_1 \cdot \vec{v}_1}{\epsilon_d} + \right. \\
& \frac{48}{5} \log\left(\frac{r}{R_\theta}\right) \hat{n} \cdot \vec{v}_1 \vec{S}_1 \times \vec{v}_1 \cdot \vec{v}_2 - 48 \log\left(\frac{r}{R_\theta}\right) \hat{n} \cdot \vec{v}_2 \hat{n} \cdot \vec{v}_1 \hat{n} \times \vec{S}_1 \cdot \vec{v}_1 + \frac{48}{5} \log\left(\frac{r}{R_\theta}\right) \vec{v}_1 \cdot \vec{v}_2 \hat{n} \times \vec{S}_1 \cdot \vec{v}_1 - \\
& \left. \frac{92}{25} \hat{n} \cdot \vec{v}_1 \vec{S}_1 \times \vec{v}_1 \cdot \vec{v}_2 + 32 \hat{n} \cdot \vec{v}_2 \hat{n} \cdot \vec{v}_1 \hat{n} \times \vec{S}_1 \cdot \vec{v}_1 + \frac{28}{25} \vec{v}_1 \cdot \vec{v}_2 \hat{n} \times \vec{S}_1 \cdot \vec{v}_1 \right\}
\end{aligned}$$

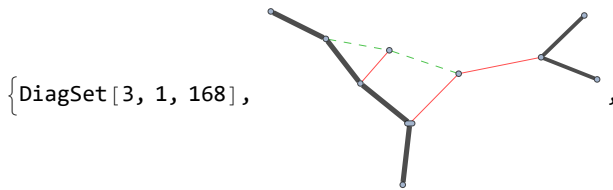

$$\begin{aligned}
& \frac{1}{r^3} G^3 m_1^2 m_2 \left( \frac{8 \hat{n} \cdot \vec{v}_1 \hat{n} \times \vec{S}_1 \cdot \vec{a}_1 + \frac{8}{3} \vec{S}_1 \times \vec{v}_1 \cdot \vec{a}_1 + 8 \hat{n} \cdot \vec{v}_1 \hat{n} \times \vec{S}_1 \cdot \vec{v}_1}{\epsilon_d} - 24 \log\left(\frac{r}{R_\theta}\right) \hat{n} \cdot \vec{v}_1 \hat{n} \times \vec{S}_1 \cdot \vec{a}_1 + \right. \\
& \left. 8 \hat{n} \cdot \vec{v}_1 \hat{n} \times \vec{S}_1 \cdot \vec{a}_1 - 8 \log\left(\frac{r}{R_\theta}\right) \vec{S}_1 \times \vec{v}_1 \cdot \vec{a}_1 - 24 \log\left(\frac{r}{R_\theta}\right) \hat{n} \cdot \vec{v}_1 \hat{n} \times \vec{S}_1 \cdot \vec{v}_1 + 8 \hat{n} \cdot \vec{v}_1 \hat{n} \times \vec{S}_1 \cdot \vec{v}_1 \right) + \frac{1}{r^4} \\
& G^3 m_1^2 m_2 \left( \frac{1}{\epsilon_d} \left( -24 (\hat{n} \cdot \vec{v}_1)^2 \hat{n} \times \vec{S}_1 \cdot \vec{v}_1 + \frac{24}{5} \hat{n} \cdot \vec{v}_1 \vec{S}_1 \times \vec{v}_1 \cdot \vec{v}_2 - 24 \hat{n} \cdot \vec{v}_2 \hat{n} \cdot \vec{v}_1 \hat{n} \times \vec{S}_1 \cdot \vec{v}_1 + \frac{24}{5} \vec{v}_1 \cdot \vec{v}_1 \hat{n} \times \vec{S}_1 \cdot \vec{v}_1 + \right. \right. \\
& \left. \frac{24}{5} \vec{v}_1 \cdot \vec{v}_2 \hat{n} \times \vec{S}_1 \cdot \vec{v}_1 \right) + 72 \log\left(\frac{r}{R_\theta}\right) (\hat{n} \cdot \vec{v}_1)^2 \hat{n} \times \vec{S}_1 \cdot \vec{v}_1 - \frac{72}{5} \log\left(\frac{r}{R_\theta}\right) \hat{n} \cdot \vec{v}_1 \vec{S}_1 \times \vec{v}_1 \cdot \vec{v}_2 + 72 \log\left(\frac{r}{R_\theta}\right) \hat{n} \cdot \vec{v}_2 \\
& \hat{n} \cdot \vec{v}_1 \hat{n} \times \vec{S}_1 \cdot \vec{v}_1 - \frac{72}{5} \log\left(\frac{r}{R_\theta}\right) \vec{v}_1 \cdot \vec{v}_1 \hat{n} \times \vec{S}_1 \cdot \vec{v}_1 - \frac{72}{5} \log\left(\frac{r}{R_\theta}\right) \vec{v}_1 \cdot \vec{v}_2 \hat{n} \times \vec{S}_1 \cdot \vec{v}_1 - 32 (\hat{n} \cdot \vec{v}_1)^2 \hat{n} \times \vec{S}_1 \cdot \vec{v}_1 + \\
& \left. \frac{88}{25} \hat{n} \cdot \vec{v}_1 \vec{S}_1 \times \vec{v}_1 \cdot \vec{v}_2 - 32 \hat{n} \cdot \vec{v}_2 \hat{n} \cdot \vec{v}_1 \hat{n} \times \vec{S}_1 \cdot \vec{v}_1 + \frac{88}{25} \vec{v}_1 \cdot \vec{v}_1 \hat{n} \times \vec{S}_1 \cdot \vec{v}_1 + \frac{88}{25} \vec{v}_1 \cdot \vec{v}_2 \hat{n} \times \vec{S}_1 \cdot \vec{v}_1 \right\}
\end{aligned}$$

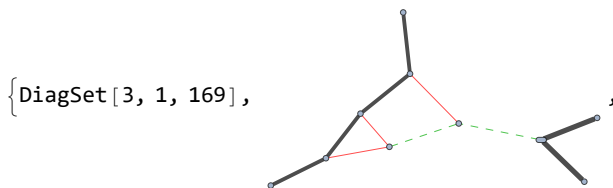

$$\begin{aligned}
& \frac{1}{r^3} G^3 m_2^3 \left( \frac{2 \hat{n} \cdot \vec{v}_2 \hat{n} \times \vec{a}_1 \cdot \vec{S}_1 - \frac{2}{3} \vec{a}_1 \times \vec{S}_1 \cdot \vec{v}_2 - 2 \hat{n} \cdot \vec{v}_2 \hat{n} \times \vec{S}_1 \cdot \vec{v}_1 + \frac{2}{3} \vec{S}_1 \times \vec{v}_1 \cdot \vec{v}_2}{\epsilon_d} - \right. \\
& 6 \log\left(\frac{r}{R_\theta}\right) \hat{n} \cdot \vec{v}_2 \hat{n} \times \vec{a}_1 \cdot \vec{S}_1 + 4 \hat{n} \cdot \vec{v}_2 \hat{n} \times \vec{a}_1 \cdot \vec{S}_1 + 2 \log\left(\frac{r}{R_\theta}\right) \vec{a}_1 \times \vec{S}_1 \cdot \vec{v}_2 + \frac{2}{3} \vec{a}_1 \times \vec{S}_1 \cdot \vec{v}_2 + \\
& \left. 6 \log\left(\frac{r}{R_\theta}\right) \hat{n} \cdot \vec{v}_2 \hat{n} \times \vec{S}_1 \cdot \vec{v}_1 - 4 \hat{n} \cdot \vec{v}_2 \hat{n} \times \vec{S}_1 \cdot \vec{v}_1 - 2 \log\left(\frac{r}{R_\theta}\right) \vec{S}_1 \times \vec{v}_1 \cdot \vec{v}_2 - \frac{2}{3} \vec{S}_1 \times \vec{v}_1 \cdot \vec{v}_2 \right) + \frac{1}{r^4}
\end{aligned}$$



$$G^3 m_2^3 \left( \frac{-2 \hat{n} \cdot \vec{v}_1 \vec{S}_1 \times \vec{v}_1 \cdot \vec{v}_2 + 10 \hat{n} \cdot \vec{v}_2 \hat{n} \cdot \vec{v}_1 \hat{n} \times \vec{S}_1 \cdot \vec{v}_1 - 2 \vec{v}_1 \cdot \vec{v}_2 \hat{n} \times \vec{S}_1 \cdot \vec{v}_1}{\in_d} + 6 \log \left( \frac{r}{R_\theta} \right) \hat{n} \cdot \vec{v}_1 \vec{S}_1 \times \vec{v}_1 \cdot \vec{v}_2 - \right. \\ \left. 30 \log \left( \frac{r}{R_\theta} \right) \hat{n} \cdot \vec{v}_2 \hat{n} \cdot \vec{v}_1 \hat{n} \times \vec{S}_1 \cdot \vec{v}_1 + 6 \log \left( \frac{r}{R_\theta} \right) \vec{v}_1 \cdot \vec{v}_2 \hat{n} \times \vec{S}_1 \cdot \vec{v}_1 - \right. \\ \left. 3 \hat{n} \cdot \vec{v}_1 \vec{S}_1 \times \vec{v}_1 \cdot \vec{v}_2 + 26 \hat{n} \cdot \vec{v}_2 \hat{n} \cdot \vec{v}_1 \hat{n} \times \vec{S}_1 \cdot \vec{v}_1 - \vec{v}_1 \cdot \vec{v}_2 \hat{n} \times \vec{S}_1 \cdot \vec{v}_1 + 9 \vec{v}_2 \cdot \vec{v}_2 \hat{n} \times \vec{S}_1 \cdot \vec{v}_2 \right) \Bigg\}$$

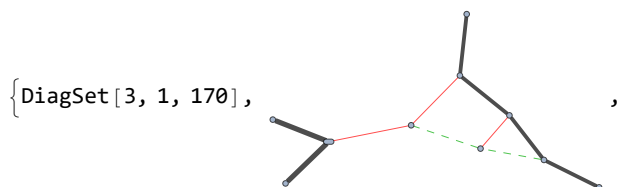

$$\frac{1}{r^3} G^3 m_2^3 \left( \frac{-8 \hat{n} \cdot \vec{v}_2 \hat{n} \times \vec{a}_1 \cdot \vec{S}_1 + \frac{8}{3} \vec{a}_1 \times \vec{S}_1 \cdot \vec{v}_2 + 8 \hat{n} \cdot \vec{v}_2 \hat{n} \times \vec{S}_1 \cdot \vec{v}_1 - \frac{8}{3} \vec{S}_1 \times \vec{v}_1 \cdot \vec{v}_2}{\epsilon_d} + 24 \log \left( \frac{r}{R_\theta} \right) \hat{n} \cdot \vec{v}_2 \hat{n} \times \vec{a}_1 \cdot \vec{S}_1 - 8 \hat{n} \cdot \vec{v}_2 \right)$$

$$\hat{n} \times \vec{a_1} \cdot \vec{S_1} - 8 \log \left( \frac{r}{R_\theta} \right) \vec{a_1} \times \vec{S_1} \cdot \vec{v_2} - 24 \log \left( \frac{r}{R_\theta} \right) \hat{n} \cdot \vec{v_2} \hat{n} \times \vec{S_1} \cdot \vec{v_1} + 8 \hat{n} \cdot \vec{v_2} \hat{n} \times \vec{S_1} \cdot \vec{v_1} + 8 \log \left( \frac{r}{R_\theta} \right) \vec{S_1} \times \vec{v_1} \cdot \vec{v_2} \Bigg) +$$

$$\begin{aligned} & \frac{1}{r^4} G^3 m^3 \left( \frac{1}{\epsilon_d} \left( -4\theta \left( \hat{n} \cdot \vec{v}_2 \right)^2 \hat{n} \times \vec{S}_1 \cdot \vec{v}_1 + 16 \hat{n} \cdot \vec{v}_2 \vec{S}_1 \times \vec{v}_1 \cdot \vec{v}_2 - 4\theta \hat{n} \cdot \vec{v}_1 \hat{n} \cdot \vec{v}_2 \hat{n} \times \vec{S}_1 \cdot \vec{v}_1 + 8 \hat{n} \cdot \vec{v}_1 \vec{S}_1 \times \vec{v}_1 \cdot \vec{v}_2 + \right. \right. \\ & \quad \left. \left. 8 \vec{v}_1 \cdot \vec{v}_2 \hat{n} \times \vec{S}_1 \cdot \vec{v}_1 + 8 \vec{v}_2 \cdot \vec{v}_2 \hat{n} \times \vec{S}_1 \cdot \vec{v}_1 \right) + 12\theta \log \left( \frac{r}{R_\theta} \right) \left( \hat{n} \cdot \vec{v}_2 \right)^2 \hat{n} \times \vec{S}_1 \cdot \vec{v}_1 - \right. \\ & \quad \left. 48 \log \left( \frac{r}{R_\theta} \right) \hat{n} \cdot \vec{v}_2 \vec{S}_1 \times \vec{v}_1 \cdot \vec{v}_2 + 12\theta \log \left( \frac{r}{R_\theta} \right) \hat{n} \cdot \vec{v}_1 \hat{n} \cdot \vec{v}_2 \hat{n} \times \vec{S}_1 \cdot \vec{v}_1 - 24 \log \left( \frac{r}{R_\theta} \right) \hat{n} \cdot \vec{v}_1 \vec{S}_1 \times \vec{v}_1 \cdot \vec{v}_2 - \right. \\ & \quad \left. 24 \log \left( \frac{r}{R_\theta} \right) \vec{v}_1 \cdot \vec{v}_2 \hat{n} \times \vec{S}_1 \cdot \vec{v}_1 - 24 \log \left( \frac{r}{R_\theta} \right) \vec{v}_2 \cdot \vec{v}_2 \hat{n} \times \vec{S}_1 \cdot \vec{v}_1 - 64 \left( \hat{n} \cdot \vec{v}_2 \right)^2 \hat{n} \times \vec{S}_1 \cdot \vec{v}_1 + 16 \hat{n} \cdot \vec{v}_2 \vec{S}_1 \times \vec{v}_1 \cdot \vec{v}_2 - \right. \\ & \quad \left. 64 \hat{n} \cdot \vec{v}_1 \hat{n} \cdot \vec{v}_2 \hat{n} \times \vec{S}_1 \cdot \vec{v}_1 + 8 \hat{n} \cdot \vec{v}_1 \vec{S}_1 \times \vec{v}_1 \cdot \vec{v}_2 + 8 \vec{v}_1 \cdot \vec{v}_2 \hat{n} \times \vec{S}_1 \cdot \vec{v}_1 + 8 \vec{v}_2 \cdot \vec{v}_2 \hat{n} \times \vec{S}_1 \cdot \vec{v}_1 \right) \Big\} \end{aligned}$$

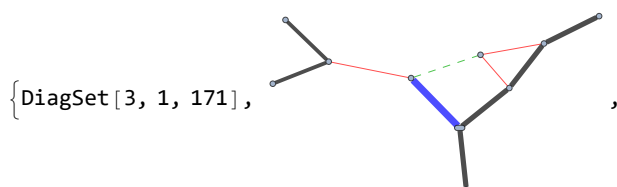

$$\frac{1}{r^3} G^3 m_1^2 m_2 \left( \frac{-\frac{1}{5} \hat{n} \cdot \vec{a}_1 \hat{n} \times \vec{S}_1 \cdot \vec{v}_1 - \frac{6}{5} \hat{n} \cdot \vec{v}_1 \hat{n} \times \vec{S}_1 \cdot \vec{a}_1 - \frac{1}{3} \vec{S}_1 \times \vec{v}_1 \cdot \vec{a}_1}{\epsilon_d} + \frac{3}{5} \log\left(\frac{r}{R_\theta}\right) \hat{n} \cdot \vec{a}_1 \hat{n} \times \vec{S}_1 \cdot \vec{v}_1 + \frac{18}{5} \log\left(\frac{r}{R_\theta}\right) \hat{n} \cdot \vec{v}_1 \right)$$

$$\hat{n} \times \vec{S_1} \cdot \vec{a_1} - \frac{17}{25} \hat{n} \cdot \vec{a_1} \hat{n} \times \vec{S_1} \cdot \vec{v_1} - \frac{67}{25} \hat{n} \cdot \vec{v_1} \hat{n} \times \vec{S_1} \cdot \vec{a_1} + \log\left(\frac{r}{R_\theta}\right) \vec{S_1} \times \vec{v_1} \cdot \vec{a_1} - \frac{1}{3} \vec{S_1} \times \vec{v_1} \cdot \vec{a_1} \Bigg) + \frac{1}{r^4} G^3 m_1^2 m_2$$

$$\begin{aligned} & \left( \frac{1}{\epsilon_d} \left( \frac{33}{7} (\hat{n} \cdot \vec{v}_1)^2 \hat{n} \times \vec{S}_1 \cdot \vec{v}_1 + \hat{n} \cdot \vec{v}_1 \vec{S}_1 \times \vec{v}_1 \cdot \vec{v}_2 - 5 \hat{n} \cdot \vec{v}_2 \hat{n} \cdot \vec{v}_1 \hat{n} \times \vec{S}_1 \cdot \vec{v}_1 - \frac{33}{35} \vec{v}_1 \cdot \vec{v}_1 \hat{n} \times \vec{S}_1 \cdot \vec{v}_1 + \vec{v}_1 \cdot \vec{v}_2 \hat{n} \times \vec{S}_1 \cdot \vec{v}_1 \right) - \right. \\ & \quad \frac{99}{7} \log \left( \frac{r}{R_\theta} \right) (\hat{n} \cdot \vec{v}_1)^2 \hat{n} \times \vec{S}_1 \cdot \vec{v}_1 - 3 \log \left( \frac{r}{R_\theta} \right) \hat{n} \cdot \vec{v}_1 \vec{S}_1 \times \vec{v}_1 \cdot \vec{v}_2 + 15 \log \left( \frac{r}{R_\theta} \right) \hat{n} \cdot \vec{v}_2 \hat{n} \cdot \vec{v}_1 \hat{n} \times \vec{S}_1 \cdot \vec{v}_1 + \\ & \quad \left. \frac{99}{35} \log \left( \frac{r}{R_\theta} \right) \vec{v}_1 \cdot \vec{v}_1 \hat{n} \times \vec{S}_1 \cdot \vec{v}_1 - 3 \log \left( \frac{r}{R_\theta} \right) \vec{v}_1 \cdot \vec{v}_2 \hat{n} \times \vec{S}_1 \cdot \vec{v}_1 + \frac{832}{49} (\hat{n} \cdot \vec{v}_1)^2 \hat{n} \times \vec{S}_1 \cdot \vec{v}_1 + \right. \end{aligned}$$

$$3 \hat{n} \cdot \vec{v}_1 \vec{S}_1 \times \vec{v}_1 \cdot \vec{v}_2 - 18 \hat{n} \cdot \vec{v}_2 \hat{n} \cdot \vec{v}_1 \hat{n} \times \vec{S}_1 \cdot \vec{v}_1 - \frac{4027 \vec{v}_1 \cdot \vec{v}_1 \hat{n} \times \vec{S}_1 \cdot \vec{v}_1}{1225} + 3 \vec{v}_1 \cdot \vec{v}_2 \hat{n} \times \vec{S}_1 \cdot \vec{v}_1 \Bigg\}$$

{DiagSet[3, 1, 172], 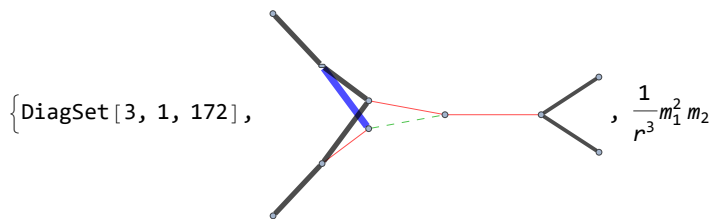 ,  $\frac{1}{r^3} m_1^2 m_2$ }

$$\begin{aligned} & \left( \log\left(\frac{r}{R_\theta}\right) \vec{S}_1 \times \vec{v}_1 \cdot \vec{a}_1 - \frac{1}{3} \vec{S}_1 \times \vec{v}_1 \cdot \vec{a}_1 - \frac{1}{3} \vec{S}_1 \times \vec{v}_1 \cdot \vec{a}_2 + \frac{33}{25} \hat{n} \times \vec{S}_1 \cdot \vec{v}_1 \hat{n} \cdot \vec{a}_1 + 2 \hat{n} \times \vec{S}_1 \cdot \vec{v}_1 \hat{n} \cdot \vec{a}_2 - \frac{17}{25} \hat{n} \times \vec{S}_1 \cdot \vec{a}_1 \hat{n} \cdot \vec{v}_1 + \right. \\ & \vec{S}_1 \times \vec{v}_1 \cdot \vec{a}_2 \log\left(\frac{r}{R_\theta}\right) - \frac{12}{5} \hat{n} \times \vec{S}_1 \cdot \vec{v}_1 \hat{n} \cdot \vec{a}_1 \log\left(\frac{r}{R_\theta}\right) - 3 \hat{n} \times \vec{S}_1 \cdot \vec{v}_1 \hat{n} \cdot \vec{a}_2 \log\left(\frac{r}{R_\theta}\right) + \frac{3}{5} \hat{n} \times \vec{S}_1 \cdot \vec{a}_1 \hat{n} \cdot \vec{v}_1 \log\left(\frac{r}{R_\theta}\right) + \\ & \left. \frac{1}{\epsilon_d} \left( -\frac{1}{3} \vec{S}_1 \times \vec{v}_1 \cdot \vec{a}_1 - \frac{1}{3} \vec{S}_1 \times \vec{v}_1 \cdot \vec{a}_2 + \frac{4}{5} \hat{n} \times \vec{S}_1 \cdot \vec{v}_1 \hat{n} \cdot \vec{a}_1 + \hat{n} \times \vec{S}_1 \cdot \vec{v}_1 \hat{n} \cdot \vec{a}_2 - \frac{1}{5} \hat{n} \times \vec{S}_1 \cdot \vec{a}_1 \hat{n} \cdot \vec{v}_1 \right) \right) G^3 + \frac{1}{r^4} \\ & m_1^2 m_2 \left( -7 \hat{n} \times \vec{S}_1 \cdot \vec{v}_1 (\hat{n} \cdot \vec{v}_1)^2 + 12 \hat{n} \times \vec{S}_1 \cdot \vec{v}_1 \log\left(\frac{r}{R_\theta}\right) (\hat{n} \cdot \vec{v}_1)^2 + \frac{41}{25} \vec{S}_1 \times \vec{v}_1 \cdot \vec{v}_2 \hat{n} \cdot \vec{v}_1 - 10 \hat{n} \times \vec{S}_1 \cdot \vec{v}_1 \hat{n} \cdot \vec{v}_2 \hat{n} \cdot \vec{v}_1 - \right. \\ & \frac{9}{5} \vec{S}_1 \times \vec{v}_1 \cdot \vec{v}_2 \log\left(\frac{r}{R_\theta}\right) \hat{n} \cdot \vec{v}_1 + 9 \hat{n} \times \vec{S}_1 \cdot \vec{v}_1 \hat{n} \cdot \vec{v}_2 \log\left(\frac{r}{R_\theta}\right) \hat{n} \cdot \vec{v}_1 + 13 \hat{n} \times \vec{S}_1 \cdot \vec{v}_1 (\hat{n} \cdot \vec{v}_2)^2 - 4 \vec{S}_1 \times \vec{v}_1 \cdot \vec{v}_2 \hat{n} \cdot \vec{v}_2 + \\ & \frac{23}{25} \hat{n} \times \vec{S}_1 \cdot \vec{v}_1 \vec{v}_1 \cdot \vec{v}_1 + \frac{41}{25} \hat{n} \times \vec{S}_1 \cdot \vec{v}_1 \vec{v}_1 \cdot \vec{v}_2 - 2 \hat{n} \times \vec{S}_1 \cdot \vec{v}_1 \vec{v}_2 \cdot \vec{v}_2 - 15 \hat{n} \times \vec{S}_1 \cdot \vec{v}_1 (\hat{n} \cdot \vec{v}_2)^2 \log\left(\frac{r}{R_\theta}\right) + \\ & 6 \vec{S}_1 \times \vec{v}_1 \cdot \vec{v}_2 \hat{n} \cdot \vec{v}_2 \log\left(\frac{r}{R_\theta}\right) - \frac{12}{5} \hat{n} \times \vec{S}_1 \cdot \vec{v}_1 \vec{v}_1 \cdot \vec{v}_1 \log\left(\frac{r}{R_\theta}\right) - \frac{9}{5} \hat{n} \times \vec{S}_1 \cdot \vec{v}_1 \vec{v}_1 \cdot \vec{v}_2 \log\left(\frac{r}{R_\theta}\right) + \\ & 3 \hat{n} \times \vec{S}_1 \cdot \vec{v}_1 \vec{v}_2 \cdot \vec{v}_2 \log\left(\frac{r}{R_\theta}\right) + \frac{1}{\epsilon_d} \left( -4 \hat{n} \times \vec{S}_1 \cdot \vec{v}_1 (\hat{n} \cdot \vec{v}_1)^2 + \frac{3}{5} \vec{S}_1 \times \vec{v}_1 \cdot \vec{v}_2 \hat{n} \cdot \vec{v}_1 - 3 \hat{n} \times \vec{S}_1 \cdot \vec{v}_1 \hat{n} \cdot \vec{v}_2 \hat{n} \cdot \vec{v}_1 + \right. \\ & \left. \left. 5 \hat{n} \times \vec{S}_1 \cdot \vec{v}_1 (\hat{n} \cdot \vec{v}_2)^2 - 2 \vec{S}_1 \times \vec{v}_1 \cdot \vec{v}_2 \hat{n} \cdot \vec{v}_2 + \frac{4}{5} \hat{n} \times \vec{S}_1 \cdot \vec{v}_1 \vec{v}_1 \cdot \vec{v}_1 + \frac{3}{5} \hat{n} \times \vec{S}_1 \cdot \vec{v}_1 \vec{v}_1 \cdot \vec{v}_2 - \hat{n} \times \vec{S}_1 \cdot \vec{v}_1 \vec{v}_2 \cdot \vec{v}_2 \right) \right) G^3 \Bigg\} \end{aligned}$$

{DiagSet[3, 1, 173], 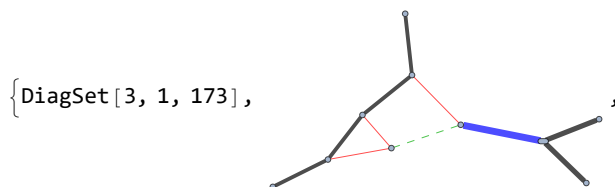 ,

$$\begin{aligned} & \frac{1}{r^3} G^3 m_2^3 \left( \frac{\frac{2}{5} \hat{n} \cdot \vec{a}_2 \hat{n} \times \vec{S}_1 \cdot \vec{v}_1 + \frac{3}{5} \hat{n} \cdot \vec{v}_1 \hat{n} \times \vec{a}_2 \cdot \vec{S}_1 - \frac{1}{3} \vec{a}_2 \times \vec{S}_1 \cdot \vec{v}_1}{\epsilon_d} - \frac{6}{5} \log\left(\frac{r}{R_\theta}\right) \hat{n} \cdot \vec{a}_2 \hat{n} \times \vec{S}_1 \cdot \vec{v}_1 - \right. \\ & \left. \frac{9}{5} \log\left(\frac{r}{R_\theta}\right) \hat{n} \cdot \vec{v}_1 \hat{n} \times \vec{a}_2 \cdot \vec{S}_1 + \frac{34}{25} \hat{n} \cdot \vec{a}_2 \hat{n} \times \vec{S}_1 \cdot \vec{v}_1 + \frac{16}{25} \hat{n} \cdot \vec{v}_1 \hat{n} \times \vec{a}_2 \cdot \vec{S}_1 + \log\left(\frac{r}{R_\theta}\right) \vec{a}_2 \times \vec{S}_1 \cdot \vec{v}_1 - \frac{1}{3} \vec{a}_2 \times \vec{S}_1 \cdot \vec{v}_1 \right) + \\ & \frac{1}{r^4} G^3 m_2^3 \left( \frac{2 (\hat{n} \cdot \vec{v}_2)^2 \hat{n} \times \vec{S}_1 \cdot \vec{v}_1 - \frac{4}{5} \hat{n} \cdot \vec{v}_2 \vec{S}_1 \times \vec{v}_1 \cdot \vec{v}_2 - \frac{2}{5} \vec{v}_2 \cdot \vec{v}_2 \hat{n} \times \vec{S}_1 \cdot \vec{v}_1}{\epsilon_d} - 6 \log\left(\frac{r}{R_\theta}\right) (\hat{n} \cdot \vec{v}_2)^2 \hat{n} \times \vec{S}_1 \cdot \vec{v}_1 + \right. \\ & \left. \frac{12}{5} \log\left(\frac{r}{R_\theta}\right) \hat{n} \cdot \vec{v}_2 \vec{S}_1 \times \vec{v}_1 \cdot \vec{v}_2 + \frac{6}{5} \log\left(\frac{r}{R_\theta}\right) \vec{v}_2 \cdot \vec{v}_2 \hat{n} \times \vec{S}_1 \cdot \vec{v}_1 + \right. \\ & \left. 8 (\hat{n} \cdot \vec{v}_2)^2 \hat{n} \times \vec{S}_1 \cdot \vec{v}_1 - \frac{68}{25} \hat{n} \cdot \vec{v}_2 \vec{S}_1 \times \vec{v}_1 \cdot \vec{v}_2 - \frac{34}{25} \vec{v}_2 \cdot \vec{v}_2 \hat{n} \times \vec{S}_1 \cdot \vec{v}_1 \right) \Bigg\} \end{aligned}$$

{DiagSet[3, 1, 174],

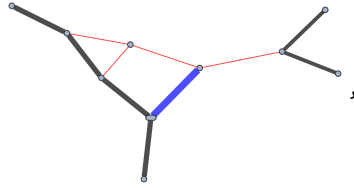

$$\frac{1}{r^3} G^3 m_1^2 m_2 \left( \frac{\frac{14}{5} \hat{n} \cdot \vec{a}_1 \hat{n} \times \vec{S}_1 \cdot \vec{v}_1 + \frac{4}{5} \hat{n} \cdot \vec{v}_1 \hat{n} \times \vec{S}_1 \cdot \vec{a}_1 - \frac{2}{3} \vec{S}_1 \times \vec{v}_1 \cdot \vec{a}_1 + \frac{18}{5} \hat{n} \cdot \vec{v}_1 \hat{n} \times \vec{S}_1 \cdot \vec{v}_1}{\epsilon_d} - \right.$$

$$\frac{42}{5} \log\left(\frac{r}{R_\theta}\right) \hat{n} \cdot \vec{a}_1 \hat{n} \times \vec{S}_1 \cdot \vec{v}_1 - \frac{12}{5} \log\left(\frac{r}{R_\theta}\right) \hat{n} \cdot \vec{v}_1 \hat{n} \times \vec{S}_1 \cdot \vec{a}_1 + \frac{183}{25} \hat{n} \cdot \vec{a}_1 \hat{n} \times \vec{S}_1 \cdot \vec{v}_1 + \frac{58}{25} \hat{n} \cdot \vec{v}_1 \hat{n} \times \vec{S}_1 \cdot \vec{a}_1 +$$

$$\left. 2 \log\left(\frac{r}{R_\theta}\right) \vec{S}_1 \times \vec{v}_1 \cdot \vec{a}_1 - \vec{S}_1 \times \vec{v}_1 \cdot \vec{a}_1 - \frac{54}{5} \log\left(\frac{r}{R_\theta}\right) \hat{n} \cdot \vec{v}_1 \hat{n} \times \vec{S}_1 \cdot \vec{v}_1 + \frac{241}{25} \hat{n} \cdot \vec{v}_1 \hat{n} \times \vec{S}_1 \cdot \vec{v}_1 \right) + \frac{1}{r^4}$$

$$G^3 m_1^2 m_2 \left( \frac{1}{\epsilon_d} \left( -5 (\hat{n} \cdot \vec{v}_1)^2 \hat{n} \times \vec{S}_1 \cdot \vec{v}_1 - \frac{18}{5} \hat{n} \cdot \vec{v}_1 \vec{S}_1 \times \vec{v}_1 \cdot \vec{v}_2 + 18 \hat{n} \cdot \vec{v}_2 \hat{n} \cdot \vec{v}_1 \hat{n} \times \vec{S}_1 \cdot \vec{v}_1 + \vec{v}_1 \cdot \vec{v}_1 \hat{n} \times \vec{S}_1 \cdot \vec{v}_1 - \right.$$

$$\frac{18}{5} \vec{v}_1 \cdot \vec{v}_2 \hat{n} \times \vec{S}_1 \cdot \vec{v}_1 \right) + 15 \log\left(\frac{r}{R_\theta}\right) (\hat{n} \cdot \vec{v}_1)^2 \hat{n} \times \vec{S}_1 \cdot \vec{v}_1 + \frac{54}{5} \log\left(\frac{r}{R_\theta}\right) \hat{n} \cdot \vec{v}_1 \vec{S}_1 \times \vec{v}_1 \cdot \vec{v}_2 - 54 \log\left(\frac{r}{R_\theta}\right) \hat{n} \cdot \vec{v}_2$$

$$\hat{n} \cdot \vec{v}_1 \hat{n} \times \vec{S}_1 \cdot \vec{v}_1 - 3 \log\left(\frac{r}{R_\theta}\right) \vec{v}_1 \cdot \vec{v}_1 \hat{n} \times \vec{S}_1 \cdot \vec{v}_1 + \frac{54}{5} \log\left(\frac{r}{R_\theta}\right) \vec{v}_1 \cdot \vec{v}_2 \hat{n} \times \vec{S}_1 \cdot \vec{v}_1 - 14 (\hat{n} \cdot \vec{v}_1)^2 \hat{n} \times \vec{S}_1 \cdot \vec{v}_1 -$$

$$\left. \frac{241}{25} \hat{n} \cdot \vec{v}_1 \vec{S}_1 \times \vec{v}_1 \cdot \vec{v}_2 + 59 \hat{n} \cdot \vec{v}_2 \hat{n} \cdot \vec{v}_1 \hat{n} \times \vec{S}_1 \cdot \vec{v}_1 + \frac{7}{5} \vec{v}_1 \cdot \vec{v}_1 \hat{n} \times \vec{S}_1 \cdot \vec{v}_1 - \frac{241}{25} \vec{v}_1 \cdot \vec{v}_2 \hat{n} \times \vec{S}_1 \cdot \vec{v}_1 \right) \}$$

{DiagSet[3, 1, 175],

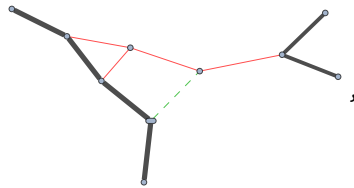

$$\frac{m_1^2 m_2 \left( -2 \log\left(\frac{r}{R_\theta}\right) \hat{n} \times \vec{S}_1 \cdot \vec{a}_1 + \frac{2 \hat{n} \times \vec{S}_1 \cdot \vec{a}_1}{3 \epsilon_d} + \hat{n} \times \vec{S}_1 \cdot \vec{a}_1 \right) G^3}{r^2} + \frac{1}{r^3} m_1^2 m_2$$

$$\left( -2 \log\left(\frac{r}{R_\theta}\right) \vec{S}_1 \times \vec{v}_1 \cdot \vec{v}_2 + \vec{S}_1 \times \vec{v}_1 \cdot \vec{v}_2 - \vec{S}_1 \times \vec{a}_1 \cdot \vec{v}_2 - \vec{S}_1 \times \vec{v}_1 \cdot \vec{a}_1 + \vec{S}_1 \times \vec{v}_1 \cdot \vec{a}_2 + \frac{41}{25} \hat{n} \times \vec{S}_1 \cdot \vec{v}_1 \hat{n} \cdot \vec{a}_1 - 5 \hat{n} \times \vec{S}_1 \cdot \vec{v}_1 \hat{n} \cdot \vec{a}_2 - \right.$$

$$\frac{116}{25} \hat{n} \times \vec{S}_1 \cdot \vec{v}_1 \hat{n} \cdot \vec{v}_1 - \frac{84}{25} \hat{n} \times \vec{S}_1 \cdot \vec{a}_1 \hat{n} \cdot \vec{v}_1 - 5 \hat{n} \times \vec{S}_1 \cdot \vec{v}_1 \hat{n} \cdot \vec{v}_2 + 5 \hat{n} \times \vec{S}_1 \cdot \vec{a}_1 \hat{n} \cdot \vec{v}_2 + 2 \vec{S}_1 \times \vec{a}_1 \cdot \vec{v}_2 \log\left(\frac{r}{R_\theta}\right) +$$

$$2 \vec{S}_1 \times \vec{v}_1 \cdot \vec{a}_1 \log\left(\frac{r}{R_\theta}\right) - 2 \vec{S}_1 \times \vec{v}_1 \cdot \vec{a}_2 \log\left(\frac{r}{R_\theta}\right) - \frac{9}{5} \hat{n} \times \vec{S}_1 \cdot \vec{v}_1 \hat{n} \cdot \vec{a}_1 \log\left(\frac{r}{R_\theta}\right) + 6 \hat{n} \times \vec{S}_1 \cdot \vec{v}_1 \hat{n} \cdot \vec{a}_2 \log\left(\frac{r}{R_\theta}\right) +$$

$$\frac{24}{5} \hat{n} \times \vec{S}_1 \cdot \vec{v}_1 \hat{n} \cdot \vec{v}_1 \log\left(\frac{r}{R_\theta}\right) + \frac{21}{5} \hat{n} \times \vec{S}_1 \cdot \vec{a}_1 \hat{n} \cdot \vec{v}_1 \log\left(\frac{r}{R_\theta}\right) + 6 \hat{n} \times \vec{S}_1 \cdot \vec{v}_1 \hat{n} \cdot \vec{v}_2 \log\left(\frac{r}{R_\theta}\right) -$$

$$6 \hat{n} \times \vec{S}_1 \cdot \vec{a}_1 \hat{n} \cdot \vec{v}_2 \log\left(\frac{r}{R_\theta}\right) + \frac{1}{\epsilon_d} \left( \frac{2}{3} \vec{S}_1 \times \vec{v}_1 \cdot \vec{v}_2 - \frac{2}{3} \vec{S}_1 \times \vec{a}_1 \cdot \vec{v}_2 - \frac{2}{3} \vec{S}_1 \times \vec{v}_1 \cdot \vec{a}_1 + \frac{2}{3} \vec{S}_1 \times \vec{v}_1 \cdot \vec{a}_2 + \frac{3}{5} \hat{n} \times \vec{S}_1 \cdot \vec{v}_1 \hat{n} \cdot \vec{a}_1 - \right.$$

$$\left. 2 \hat{n} \times \vec{S}_1 \cdot \vec{v}_1 \hat{n} \cdot \vec{a}_2 - \frac{8}{5} \hat{n} \times \vec{S}_1 \cdot \vec{v}_1 \hat{n} \cdot \vec{v}_1 - \frac{7}{5} \hat{n} \times \vec{S}_1 \cdot \vec{a}_1 \hat{n} \cdot \vec{v}_1 - 2 \hat{n} \times \vec{S}_1 \cdot \vec{v}_1 \hat{n} \cdot \vec{v}_2 + 2 \hat{n} \times \vec{S}_1 \cdot \vec{a}_1 \hat{n} \cdot \vec{v}_2 \right) \Big) G^3 + \frac{1}{r^4}$$

$$m_1^2 m_2 \left( 7 \hat{n} \times \vec{S}_1 \cdot \vec{v}_1 (\hat{n} \cdot \vec{v}_1)^2 - 6 \hat{n} \times \vec{S}_1 \cdot \vec{v}_1 \log\left(\frac{r}{R_\theta}\right) (\hat{n} \cdot \vec{v}_1)^2 + \frac{18}{5} \vec{S}_1 \times \vec{v}_1 \cdot \vec{v}_2 \hat{n} \cdot \vec{v}_1 - 21 \hat{n} \times \vec{S}_1 \cdot \vec{v}_1 \hat{n} \cdot \vec{v}_2 \hat{n} \cdot \vec{v}_1 - \right.$$

$$\left. 3 \vec{S}_1 \times \vec{v}_1 \cdot \vec{v}_2 \log\left(\frac{r}{R_\theta}\right) \hat{n} \cdot \vec{v}_1 + 15 \hat{n} \times \vec{S}_1 \cdot \vec{v}_1 \hat{n} \cdot \vec{v}_2 \log\left(\frac{r}{R_\theta}\right) \hat{n} \cdot \vec{v}_1 - 31 \hat{n} \times \vec{S}_1 \cdot \vec{v}_1 (\hat{n} \cdot \vec{v}_2)^2 + 10 \vec{S}_1 \times \vec{v}_1 \cdot \vec{v}_2 \hat{n} \cdot \vec{v}_2 - \right.$$

$$\begin{aligned} & \frac{9}{25} \hat{n} \times \vec{S}_1 \cdot \vec{v}_1 \vec{v}_1 \cdot \vec{v}_1 + \frac{18}{5} \hat{n} \times \vec{S}_1 \cdot \vec{v}_1 \vec{v}_1 \cdot \vec{v}_2 + 5 \hat{n} \times \vec{S}_1 \cdot \vec{v}_1 \vec{v}_2 \cdot \vec{v}_2 + 30 \hat{n} \times \vec{S}_1 \cdot \vec{v}_1 (\hat{n} \cdot \vec{v}_2)^2 \log\left(\frac{r}{R_\theta}\right) - \\ & 12 \vec{S}_1 \times \vec{v}_1 \cdot \vec{v}_2 \hat{n} \cdot \vec{v}_2 \log\left(\frac{r}{R_\theta}\right) + \frac{6}{5} \hat{n} \times \vec{S}_1 \cdot \vec{v}_1 \vec{v}_1 \cdot \vec{v}_1 \log\left(\frac{r}{R_\theta}\right) - 3 \hat{n} \times \vec{S}_1 \cdot \vec{v}_1 \vec{v}_1 \cdot \vec{v}_2 \log\left(\frac{r}{R_\theta}\right) - \\ & 6 \hat{n} \times \vec{S}_1 \cdot \vec{v}_1 \vec{v}_2 \cdot \vec{v}_2 \log\left(\frac{r}{R_\theta}\right) + \frac{1}{\epsilon_d} \left( 2 \hat{n} \times \vec{S}_1 \cdot \vec{v}_1 (\hat{n} \cdot \vec{v}_1)^2 + \vec{S}_1 \times \vec{v}_1 \cdot \vec{v}_2 \hat{n} \cdot \vec{v}_1 - 5 \hat{n} \times \vec{S}_1 \cdot \vec{v}_1 \hat{n} \cdot \vec{v}_2 \hat{n} \cdot \vec{v}_1 - \right. \\ & \left. 10 \hat{n} \times \vec{S}_1 \cdot \vec{v}_1 (\hat{n} \cdot \vec{v}_2)^2 + 4 \vec{S}_1 \times \vec{v}_1 \cdot \vec{v}_2 \hat{n} \cdot \vec{v}_2 - \frac{2}{5} \hat{n} \times \vec{S}_1 \cdot \vec{v}_1 \vec{v}_1 \cdot \vec{v}_1 + \hat{n} \times \vec{S}_1 \cdot \vec{v}_1 \vec{v}_1 \cdot \vec{v}_2 + 2 \hat{n} \times \vec{S}_1 \cdot \vec{v}_1 \vec{v}_2 \cdot \vec{v}_2 \right) \Big) G^3 \Big\} \end{aligned}$$

{DiagSet[3, 1, 176],

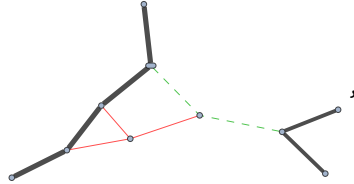

$$\begin{aligned} & \frac{1}{r^3} m_1^2 m_2 \left( \frac{32}{5} \log\left(\frac{r}{R_\theta}\right) \vec{S}_1 \times \vec{v}_1 \cdot \vec{v}_2 - \frac{224}{75} \vec{S}_1 \times \vec{v}_1 \cdot \vec{v}_2 - \frac{224}{75} \vec{S}_1 \times \vec{v}_1 \cdot \vec{a}_2 + \frac{208}{25} \hat{n} \times \vec{S}_1 \cdot \vec{v}_1 \hat{n} \cdot \vec{a}_2 + \frac{64}{25} \hat{n} \times \vec{S}_1 \cdot \vec{v}_2 \hat{n} \cdot \vec{v}_1 + \right. \\ & \frac{64}{25} \hat{n} \times \vec{S}_1 \cdot \vec{a}_2 \hat{n} \cdot \vec{v}_1 + \frac{208}{25} \hat{n} \times \vec{S}_1 \cdot \vec{v}_1 \hat{n} \cdot \vec{v}_2 + \frac{32}{5} \vec{S}_1 \times \vec{v}_1 \cdot \vec{a}_2 \log\left(\frac{r}{R_\theta}\right) - \frac{72}{5} \hat{n} \times \vec{S}_1 \cdot \vec{v}_1 \hat{n} \cdot \vec{a}_2 \log\left(\frac{r}{R_\theta}\right) + \\ & \frac{24}{5} \hat{n} \times \vec{S}_1 \cdot \vec{v}_2 \hat{n} \cdot \vec{v}_1 \log\left(\frac{r}{R_\theta}\right) + \frac{24}{5} \hat{n} \times \vec{S}_1 \cdot \vec{a}_2 \hat{n} \cdot \vec{v}_1 \log\left(\frac{r}{R_\theta}\right) - \frac{72}{5} \hat{n} \times \vec{S}_1 \cdot \vec{v}_1 \hat{n} \cdot \vec{v}_2 \log\left(\frac{r}{R_\theta}\right) + \frac{1}{\epsilon_d} \left( -\frac{32}{15} \vec{S}_1 \times \vec{v}_1 \cdot \vec{v}_2 - \right. \\ & \left. \frac{32}{15} \vec{S}_1 \times \vec{v}_1 \cdot \vec{a}_2 + \frac{24}{5} \hat{n} \times \vec{S}_1 \cdot \vec{v}_1 \hat{n} \cdot \vec{a}_2 - \frac{8}{5} \hat{n} \times \vec{S}_1 \cdot \vec{v}_2 \hat{n} \cdot \vec{v}_1 - \frac{8}{5} \hat{n} \times \vec{S}_1 \cdot \vec{a}_2 \hat{n} \cdot \vec{v}_1 + \frac{24}{5} \hat{n} \times \vec{S}_1 \cdot \vec{v}_1 \hat{n} \cdot \vec{v}_2 \right) \Big) G^3 + \frac{1}{r^4} \\ & m_1^2 m_2 \left( -10 \hat{n} \times \vec{S}_1 \cdot \vec{v}_2 (\hat{n} \cdot \vec{v}_1)^2 - 12 \hat{n} \times \vec{S}_1 \cdot \vec{v}_2 \log\left(\frac{r}{R_\theta}\right) (\hat{n} \cdot \vec{v}_1)^2 + \frac{2}{5} \vec{S}_1 \times \vec{v}_1 \cdot \vec{v}_2 \hat{n} \cdot \vec{v}_1 - 22 \hat{n} \times \vec{S}_1 \cdot \vec{v}_1 \hat{n} \cdot \vec{v}_2 \hat{n} \cdot \vec{v}_1 + \right. \\ & 8 \hat{n} \times \vec{S}_1 \cdot \vec{v}_2 \hat{n} \cdot \vec{v}_2 \hat{n} \cdot \vec{v}_1 - 12 \vec{S}_1 \times \vec{v}_1 \cdot \vec{v}_2 \log\left(\frac{r}{R_\theta}\right) \hat{n} \cdot \vec{v}_1 + 36 \hat{n} \times \vec{S}_1 \cdot \vec{v}_1 \hat{n} \cdot \vec{v}_2 \log\left(\frac{r}{R_\theta}\right) \hat{n} \cdot \vec{v}_1 + \\ & 24 \hat{n} \times \vec{S}_1 \cdot \vec{v}_2 \hat{n} \cdot \vec{v}_2 \log\left(\frac{r}{R_\theta}\right) \hat{n} \cdot \vec{v}_1 + 56 \hat{n} \times \vec{S}_1 \cdot \vec{v}_1 (\hat{n} \cdot \vec{v}_2)^2 - \frac{592}{25} \vec{S}_1 \times \vec{v}_1 \cdot \vec{v}_2 \hat{n} \cdot \vec{v}_2 - \frac{18}{25} \hat{n} \times \vec{S}_1 \cdot \vec{v}_2 \vec{v}_1 \cdot \vec{v}_1 + \\ & \frac{134}{25} \hat{n} \times \vec{S}_1 \cdot \vec{v}_1 \vec{v}_1 \cdot \vec{v}_2 - \frac{64}{25} \hat{n} \times \vec{S}_1 \cdot \vec{v}_2 \vec{v}_1 \cdot \vec{v}_2 - \frac{208}{25} \hat{n} \times \vec{S}_1 \cdot \vec{v}_1 \vec{v}_2 \cdot \vec{v}_2 - 72 \hat{n} \times \vec{S}_1 \cdot \vec{v}_1 (\hat{n} \cdot \vec{v}_2)^2 \log\left(\frac{r}{R_\theta}\right) + \\ & \frac{168}{5} \vec{S}_1 \times \vec{v}_1 \cdot \vec{v}_2 \hat{n} \cdot \vec{v}_2 \log\left(\frac{r}{R_\theta}\right) + \frac{12}{5} \hat{n} \times \vec{S}_1 \cdot \vec{v}_2 \vec{v}_1 \cdot \vec{v}_1 \log\left(\frac{r}{R_\theta}\right) - \frac{36}{5} \hat{n} \times \vec{S}_1 \cdot \vec{v}_1 \vec{v}_1 \cdot \vec{v}_2 \log\left(\frac{r}{R_\theta}\right) - \\ & \frac{24}{5} \hat{n} \times \vec{S}_1 \cdot \vec{v}_2 \vec{v}_1 \cdot \vec{v}_2 \log\left(\frac{r}{R_\theta}\right) + \frac{72}{5} \hat{n} \times \vec{S}_1 \cdot \vec{v}_1 \vec{v}_2 \cdot \vec{v}_2 \log\left(\frac{r}{R_\theta}\right) + \frac{1}{\epsilon_d} \left( 4 \hat{n} \times \vec{S}_1 \cdot \vec{v}_2 (\hat{n} \cdot \vec{v}_1)^2 + 4 \vec{S}_1 \times \vec{v}_1 \cdot \vec{v}_2 \hat{n} \cdot \vec{v}_1 - \right. \\ & \left. 12 \hat{n} \times \vec{S}_1 \cdot \vec{v}_1 \hat{n} \cdot \vec{v}_2 \hat{n} \cdot \vec{v}_1 - 8 \hat{n} \times \vec{S}_1 \cdot \vec{v}_2 \hat{n} \cdot \vec{v}_2 \hat{n} \cdot \vec{v}_1 + 24 \hat{n} \times \vec{S}_1 \cdot \vec{v}_1 (\hat{n} \cdot \vec{v}_2)^2 - \frac{56}{5} \vec{S}_1 \times \vec{v}_1 \cdot \vec{v}_2 \hat{n} \cdot \vec{v}_2 - \right. \\ & \left. \frac{4}{5} \hat{n} \times \vec{S}_1 \cdot \vec{v}_2 \vec{v}_1 \cdot \vec{v}_1 + \frac{12}{5} \hat{n} \times \vec{S}_1 \cdot \vec{v}_1 \vec{v}_1 \cdot \vec{v}_2 + \frac{8}{5} \hat{n} \times \vec{S}_1 \cdot \vec{v}_2 \vec{v}_1 \cdot \vec{v}_2 - \frac{24}{5} \hat{n} \times \vec{S}_1 \cdot \vec{v}_1 \vec{v}_2 \cdot \vec{v}_2 \right) \Big) G^3 \Big\} \end{aligned}$$

{DiagSet[3, 1, 177],

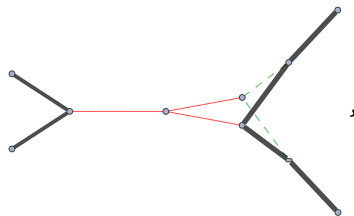

$$\begin{aligned} & \frac{1}{r^3} m_1^2 m_2 \left( -4 \log\left(\frac{r}{R_\theta}\right) \vec{S}_1 \times \vec{v}_1 \cdot \vec{v}_2 + \frac{2}{3} \vec{S}_1 \times \vec{v}_1 \cdot \vec{v}_2 + \frac{2}{3} \vec{S}_1 \times \vec{a}_1 \cdot \vec{v}_2 - \frac{2}{75} \vec{S}_1 \times \vec{v}_1 \cdot \vec{a}_1 + \frac{38}{25} \hat{n} \times \vec{S}_1 \cdot \vec{v}_1 \hat{n} \cdot \vec{v}_1 + \right. \\ & \frac{38}{25} \hat{n} \times \vec{S}_1 \cdot \vec{a}_1 \hat{n} \cdot \vec{v}_1 - 6 \hat{n} \times \vec{S}_1 \cdot \vec{v}_1 \hat{n} \cdot \vec{v}_2 - 6 \hat{n} \times \vec{S}_1 \cdot \vec{a}_1 \hat{n} \cdot \vec{v}_2 - 4 \vec{S}_1 \times \vec{a}_1 \cdot \vec{v}_2 \log\left(\frac{r}{R_\theta}\right) - \end{aligned}$$

$$\begin{aligned} & \frac{4}{5} \vec{S}_1 \times \vec{v}_1 \cdot \vec{a}_1 \log\left(\frac{r}{R_\theta}\right) - \frac{12}{5} \hat{n} \times \vec{S}_1 \cdot \vec{v}_1 \hat{n} \cdot \vec{v}_1 \log\left(\frac{r}{R_\theta}\right) - \frac{12}{5} \hat{n} \times \vec{S}_1 \cdot \vec{a}_1 \hat{n} \cdot \vec{v}_1 \log\left(\frac{r}{R_\theta}\right) + \\ & 12 \hat{n} \times \vec{S}_1 \cdot \vec{v}_1 \hat{n} \cdot \vec{v}_2 \log\left(\frac{r}{R_\theta}\right) + 12 \hat{n} \times \vec{S}_1 \cdot \vec{a}_1 \hat{n} \cdot \vec{v}_2 \log\left(\frac{r}{R_\theta}\right) + \frac{1}{\epsilon_d} \left( \frac{4}{3} \vec{S}_1 \times \vec{v}_1 \cdot \vec{v}_2 + \frac{4}{3} \vec{S}_1 \times \vec{a}_1 \cdot \vec{v}_2 + \right. \\ & \left. \frac{4}{15} \vec{S}_1 \times \vec{v}_1 \cdot \vec{a}_1 + \frac{4}{5} \hat{n} \times \vec{S}_1 \cdot \vec{v}_1 \hat{n} \cdot \vec{v}_1 + \frac{4}{5} \hat{n} \times \vec{S}_1 \cdot \vec{a}_1 \hat{n} \cdot \vec{v}_1 - 4 \hat{n} \times \vec{S}_1 \cdot \vec{v}_1 \hat{n} \cdot \vec{v}_2 - 4 \hat{n} \times \vec{S}_1 \cdot \vec{a}_1 \hat{n} \cdot \vec{v}_2 \right) \Bigg) G^3 + \frac{1}{r^4} \\ & m_1^2 m_2 \left( -\frac{288}{49} \hat{n} \times \vec{S}_1 \cdot \vec{v}_1 (\hat{n} \cdot \vec{v}_1)^2 + \frac{48}{7} \hat{n} \times \vec{S}_1 \cdot \vec{v}_1 \log\left(\frac{r}{R_\theta}\right) (\hat{n} \cdot \vec{v}_1)^2 - 6 \vec{S}_1 \times \vec{v}_1 \cdot \vec{v}_2 \hat{n} \cdot \vec{v}_1 + 42 \hat{n} \times \vec{S}_1 \cdot \vec{v}_1 \hat{n} \cdot \vec{v}_2 \hat{n} \cdot \vec{v}_1 + \right. \\ & 12 \vec{S}_1 \times \vec{v}_1 \cdot \vec{v}_2 \log\left(\frac{r}{R_\theta}\right) \hat{n} \cdot \vec{v}_1 - 60 \hat{n} \times \vec{S}_1 \cdot \vec{v}_1 \hat{n} \cdot \vec{v}_2 \log\left(\frac{r}{R_\theta}\right) \hat{n} \cdot \vec{v}_1 + \frac{544 \hat{n} \times \vec{S}_1 \cdot \vec{v}_1 \vec{v}_1 \cdot \vec{v}_1}{1225} - 6 \hat{n} \times \vec{S}_1 \cdot \vec{v}_1 \vec{v}_1 \cdot \vec{v}_2 - \\ & \frac{48}{35} \hat{n} \times \vec{S}_1 \cdot \vec{v}_1 \vec{v}_1 \cdot \vec{v}_1 \log\left(\frac{r}{R_\theta}\right) + 12 \hat{n} \times \vec{S}_1 \cdot \vec{v}_1 \vec{v}_1 \cdot \vec{v}_2 \log\left(\frac{r}{R_\theta}\right) + \frac{1}{\epsilon_d} \left( -\frac{16}{7} \hat{n} \times \vec{S}_1 \cdot \vec{v}_1 (\hat{n} \cdot \vec{v}_1)^2 - \right. \\ & \left. 4 \vec{S}_1 \times \vec{v}_1 \cdot \vec{v}_2 \hat{n} \cdot \vec{v}_1 + 20 \hat{n} \times \vec{S}_1 \cdot \vec{v}_1 \hat{n} \cdot \vec{v}_2 \hat{n} \cdot \vec{v}_1 + \frac{16}{35} \hat{n} \times \vec{S}_1 \cdot \vec{v}_1 \vec{v}_1 \cdot \vec{v}_1 - 4 \hat{n} \times \vec{S}_1 \cdot \vec{v}_1 \vec{v}_1 \cdot \vec{v}_2 \right) \Bigg) G^3 \Bigg\} \end{aligned}$$

{DiagSet[3, 1, 178], 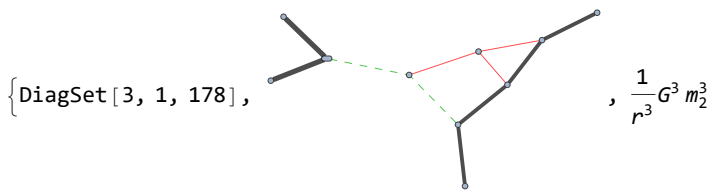 ,  $\frac{1}{r^3} G^3 m_2^3$

$$\begin{aligned} & \left( \frac{8 \hat{n} \cdot \vec{a}_2 \hat{n} \times \vec{S}_1 \cdot \vec{v}_2 + 8 \hat{n} \cdot \vec{v}_2 \hat{n} \times \vec{a}_2 \cdot \vec{S}_1 - \frac{16}{3} \vec{a}_2 \times \vec{S}_1 \cdot \vec{v}_2}{\epsilon_d} - 24 \log\left(\frac{r}{R_\theta}\right) \hat{n} \cdot \vec{a}_2 \hat{n} \times \vec{S}_1 \cdot \vec{v}_2 - 24 \log\left(\frac{r}{R_\theta}\right) \hat{n} \cdot \vec{v}_2 \hat{n} \times \vec{a}_2 \cdot \vec{S}_1 + \right. \\ & 16 \hat{n} \cdot \vec{a}_2 \hat{n} \times \vec{S}_1 \cdot \vec{v}_2 + 32 \hat{n} \cdot \vec{v}_2 \hat{n} \times \vec{a}_2 \cdot \vec{S}_1 + 16 \log\left(\frac{r}{R_\theta}\right) \vec{a}_2 \times \vec{S}_1 \cdot \vec{v}_2 - \frac{32}{3} \vec{a}_2 \times \vec{S}_1 \cdot \vec{v}_2 - 16 \hat{n} \cdot \vec{v}_2 \hat{n} \times \vec{S}_1 \cdot \vec{v}_2 \Bigg) + \frac{1}{r^4} G^3 m_2^3 \\ & \left( -52 (\hat{n} \cdot \vec{v}_2)^2 \hat{n} \times \vec{S}_1 \cdot \vec{v}_2 + 16 \hat{n} \cdot \vec{v}_2 \vec{S}_1 \times \vec{v}_1 \cdot \vec{v}_2 + 80 \hat{n} \cdot \vec{v}_1 \hat{n} \cdot \vec{v}_2 \hat{n} \times \vec{S}_1 \cdot \vec{v}_2 - 16 \vec{v}_1 \cdot \vec{v}_2 \hat{n} \times \vec{S}_1 \cdot \vec{v}_2 + 4 \vec{v}_2 \cdot \vec{v}_2 \hat{n} \times \vec{S}_1 \cdot \vec{v}_2 \right) \Bigg\} \end{aligned}$$

{DiagSet[3, 1, 179], 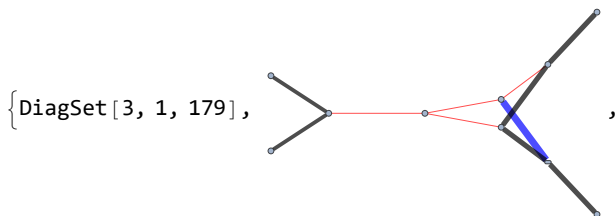 ,

$$\begin{aligned} & \frac{1}{r^3} m_1^2 m_2 \left( \frac{1}{5} \log\left(\frac{r}{R_\theta}\right) \vec{S}_1 \times \vec{v}_1 \cdot \vec{a}_1 + \frac{1}{25} \vec{S}_1 \times \vec{v}_1 \cdot \vec{a}_1 - \frac{7}{25} \hat{n} \times \vec{S}_1 \cdot \vec{v}_1 \hat{n} \cdot \vec{v}_1 - \frac{7}{25} \hat{n} \times \vec{S}_1 \cdot \vec{a}_1 \hat{n} \cdot \vec{v}_1 + \hat{n} \times \vec{S}_1 \cdot \vec{v}_1 \hat{n} \cdot \vec{v}_2 + \right. \\ & \hat{n} \times \vec{S}_1 \cdot \vec{a}_1 \hat{n} \cdot \vec{v}_2 + \vec{S}_1 \times \vec{v}_1 \cdot \vec{v}_2 \log\left(\frac{r}{R_\theta}\right) + \vec{S}_1 \times \vec{a}_1 \cdot \vec{v}_2 \log\left(\frac{r}{R_\theta}\right) + \frac{3}{5} \hat{n} \times \vec{S}_1 \cdot \vec{v}_1 \hat{n} \cdot \vec{v}_1 \log\left(\frac{r}{R_\theta}\right) + \\ & \frac{3}{5} \hat{n} \times \vec{S}_1 \cdot \vec{a}_1 \hat{n} \cdot \vec{v}_1 \log\left(\frac{r}{R_\theta}\right) - 3 \hat{n} \times \vec{S}_1 \cdot \vec{v}_1 \hat{n} \cdot \vec{v}_2 \log\left(\frac{r}{R_\theta}\right) - 3 \hat{n} \times \vec{S}_1 \cdot \vec{a}_1 \hat{n} \cdot \vec{v}_2 \log\left(\frac{r}{R_\theta}\right) + \frac{1}{\epsilon_d} \left( -\frac{1}{3} \vec{S}_1 \times \vec{v}_1 \cdot \vec{v}_2 - \right. \\ & \left. \frac{1}{3} \vec{S}_1 \times \vec{a}_1 \cdot \vec{v}_2 - \frac{1}{15} \vec{S}_1 \times \vec{v}_1 \cdot \vec{a}_1 - \frac{1}{5} \hat{n} \times \vec{S}_1 \cdot \vec{v}_1 \hat{n} \cdot \vec{v}_1 - \frac{1}{5} \hat{n} \times \vec{S}_1 \cdot \vec{a}_1 \hat{n} \cdot \vec{v}_1 + \hat{n} \times \vec{S}_1 \cdot \vec{v}_1 \hat{n} \cdot \vec{v}_2 + \hat{n} \times \vec{S}_1 \cdot \vec{a}_1 \hat{n} \cdot \vec{v}_2 \right) \Bigg) G^3 + \\ & \frac{1}{r^4} m_1^2 m_2 \left( \frac{58}{49} \hat{n} \times \vec{S}_1 \cdot \vec{v}_1 (\hat{n} \cdot \vec{v}_1)^2 - \frac{12}{7} \hat{n} \times \vec{S}_1 \cdot \vec{v}_1 \log\left(\frac{r}{R_\theta}\right) (\hat{n} \cdot \vec{v}_1)^2 + \vec{S}_1 \times \vec{v}_1 \cdot \vec{v}_2 \hat{n} \cdot \vec{v}_1 - 8 \hat{n} \times \vec{S}_1 \cdot \vec{v}_1 \hat{n} \cdot \vec{v}_2 \hat{n} \cdot \vec{v}_1 - \right. \\ & 3 \vec{S}_1 \times \vec{v}_1 \cdot \vec{v}_2 \log\left(\frac{r}{R_\theta}\right) \hat{n} \cdot \vec{v}_1 + 15 \hat{n} \times \vec{S}_1 \cdot \vec{v}_1 \hat{n} \cdot \vec{v}_2 \log\left(\frac{r}{R_\theta}\right) \hat{n} \cdot \vec{v}_1 - \frac{66 \hat{n} \times \vec{S}_1 \cdot \vec{v}_1 \vec{v}_1 \cdot \vec{v}_1}{1225} + \\ & \left. \hat{n} \times \vec{S}_1 \cdot \vec{v}_1 \vec{v}_1 \cdot \vec{v}_2 + \frac{12}{35} \hat{n} \times \vec{S}_1 \cdot \vec{v}_1 \vec{v}_1 \cdot \vec{v}_1 \log\left(\frac{r}{R_\theta}\right) - 3 \hat{n} \times \vec{S}_1 \cdot \vec{v}_1 \vec{v}_1 \cdot \vec{v}_2 \log\left(\frac{r}{R_\theta}\right) + \frac{1}{\epsilon_d} \right) \end{aligned}$$

$$\left( \frac{4}{7} \hat{n} \times \vec{S}_1 \cdot \vec{v}_1 (\hat{n} \cdot \vec{v}_1)^2 + \vec{S}_1 \times \vec{v}_1 \cdot \vec{v}_2 \hat{n} \cdot \vec{v}_1 - 5 \hat{n} \times \vec{S}_1 \cdot \vec{v}_1 \hat{n} \cdot \vec{v}_2 \hat{n} \cdot \vec{v}_1 - \frac{4}{35} \hat{n} \times \vec{S}_1 \cdot \vec{v}_1 \vec{v}_1 \cdot \vec{v}_1 + \hat{n} \times \vec{S}_1 \cdot \vec{v}_1 \vec{v}_1 \cdot \vec{v}_2 \right) G^3 \Bigg\}$$

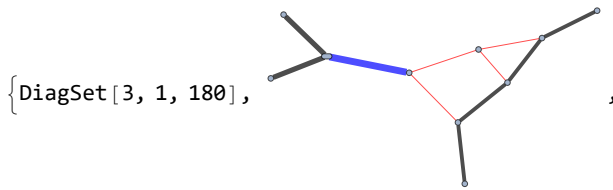

$$\begin{aligned} & \frac{1}{r^3} G^3 \left( -2 \log \left( \frac{r}{R_0} \right) \vec{S}_1 \times \vec{v}_1 \cdot \vec{v}_2 + \vec{S}_1 \times \vec{v}_1 \cdot \vec{v}_2 - \vec{a}_1 \times \vec{S}_1 \cdot \vec{v}_2 + \frac{9}{25} \hat{n} \times \vec{S}_1 \cdot \vec{v}_2 \hat{n} \cdot \vec{a}_1 + \frac{9}{25} \hat{n} \times \vec{S}_1 \cdot \vec{v}_2 \hat{n} \cdot \vec{v}_1 - \right. \\ & \frac{116}{25} \hat{n} \times \vec{S}_1 \cdot \vec{v}_1 \hat{n} \cdot \vec{v}_2 + \frac{116}{25} \hat{n} \times \vec{a}_1 \cdot \vec{S}_1 \hat{n} \cdot \vec{v}_2 + 2 \vec{a}_1 \times \vec{S}_1 \cdot \vec{v}_2 \log \left( \frac{r}{R_0} \right) - \frac{6}{5} \hat{n} \times \vec{S}_1 \cdot \vec{v}_2 \hat{n} \cdot \vec{a}_1 \log \left( \frac{r}{R_0} \right) - \\ & \frac{6}{5} \hat{n} \times \vec{S}_1 \cdot \vec{v}_2 \hat{n} \cdot \vec{v}_1 \log \left( \frac{r}{R_0} \right) + \frac{24}{5} \hat{n} \times \vec{S}_1 \cdot \vec{v}_1 \hat{n} \cdot \vec{v}_2 \log \left( \frac{r}{R_0} \right) - \frac{24}{5} \hat{n} \times \vec{a}_1 \cdot \vec{S}_1 \hat{n} \cdot \vec{v}_2 \log \left( \frac{r}{R_0} \right) + \frac{1}{\epsilon_d} \\ & \left. \left( \frac{2}{3} \vec{S}_1 \times \vec{v}_1 \cdot \vec{v}_2 - \frac{2}{3} \vec{a}_1 \times \vec{S}_1 \cdot \vec{v}_2 + \frac{2}{5} \hat{n} \times \vec{S}_1 \cdot \vec{v}_2 \hat{n} \cdot \vec{a}_1 + \frac{2}{5} \hat{n} \times \vec{S}_1 \cdot \vec{v}_2 \hat{n} \cdot \vec{v}_1 - \frac{8}{5} \hat{n} \times \vec{S}_1 \cdot \vec{v}_1 \hat{n} \cdot \vec{v}_2 + \frac{8}{5} \hat{n} \times \vec{a}_1 \cdot \vec{S}_1 \hat{n} \cdot \vec{v}_2 \right) \right) \\ & m_2^2 + \frac{1}{r^4} G^3 \left( -3 \hat{n} \times \vec{S}_1 \cdot \vec{v}_2 (\hat{n} \cdot \vec{v}_1)^2 + 6 \hat{n} \times \vec{S}_1 \cdot \vec{v}_2 \log \left( \frac{r}{R_0} \right) (\hat{n} \cdot \vec{v}_1)^2 - \frac{134}{25} \vec{S}_1 \times \vec{v}_1 \cdot \vec{v}_2 \hat{n} \cdot \vec{v}_1 + 28 \hat{n} \times \vec{S}_1 \cdot \vec{v}_1 \hat{n} \cdot \vec{v}_2 \hat{n} \cdot \vec{v}_1 + \right. \\ & 7 \hat{n} \times \vec{S}_1 \cdot \vec{v}_2 \hat{n} \cdot \vec{v}_2 \hat{n} \cdot \vec{v}_1 + \frac{36}{5} \vec{S}_1 \times \vec{v}_1 \cdot \vec{v}_2 \log \left( \frac{r}{R_0} \right) \hat{n} \cdot \vec{v}_1 - 24 \hat{n} \times \vec{S}_1 \cdot \vec{v}_1 \hat{n} \cdot \vec{v}_2 \log \left( \frac{r}{R_0} \right) \hat{n} \cdot \vec{v}_1 - \\ & 9 \hat{n} \times \vec{S}_1 \cdot \vec{v}_2 \hat{n} \cdot \vec{v}_2 \log \left( \frac{r}{R_0} \right) \hat{n} \cdot \vec{v}_1 - 14 \hat{n} \times \vec{S}_1 \cdot \vec{v}_1 (\hat{n} \cdot \vec{v}_2)^2 + \frac{142}{25} \vec{S}_1 \times \vec{v}_1 \cdot \vec{v}_2 \hat{n} \cdot \vec{v}_2 + \frac{9}{25} \hat{n} \times \vec{S}_1 \cdot \vec{v}_2 \vec{v}_1 \cdot \vec{v}_1 - \\ & \frac{116}{25} \hat{n} \times \vec{S}_1 \cdot \vec{v}_1 \vec{v}_1 \cdot \vec{v}_2 - \frac{56}{25} \hat{n} \times \vec{S}_1 \cdot \vec{v}_2 \vec{v}_1 \cdot \vec{v}_2 + \frac{48}{25} \hat{n} \times \vec{S}_1 \cdot \vec{v}_1 \vec{v}_2 \cdot \vec{v}_2 + 12 \hat{n} \times \vec{S}_1 \cdot \vec{v}_1 (\hat{n} \cdot \vec{v}_2)^2 \log \left( \frac{r}{R_0} \right) - \\ & \frac{33}{5} \vec{S}_1 \times \vec{v}_1 \cdot \vec{v}_2 \hat{n} \cdot \vec{v}_2 \log \left( \frac{r}{R_0} \right) - \frac{6}{5} \hat{n} \times \vec{S}_1 \cdot \vec{v}_2 \vec{v}_1 \cdot \vec{v}_1 \log \left( \frac{r}{R_0} \right) + \frac{24}{5} \hat{n} \times \vec{S}_1 \cdot \vec{v}_1 \vec{v}_1 \cdot \vec{v}_2 \log \left( \frac{r}{R_0} \right) + \\ & \frac{9}{5} \hat{n} \times \vec{S}_1 \cdot \vec{v}_2 \vec{v}_1 \cdot \vec{v}_2 \log \left( \frac{r}{R_0} \right) - \frac{12}{5} \hat{n} \times \vec{S}_1 \cdot \vec{v}_1 \vec{v}_2 \cdot \vec{v}_2 \log \left( \frac{r}{R_0} \right) + \frac{1}{\epsilon_d} \left( -2 \hat{n} \times \vec{S}_1 \cdot \vec{v}_2 (\hat{n} \cdot \vec{v}_1)^2 - \frac{12}{5} \vec{S}_1 \times \vec{v}_1 \cdot \vec{v}_2 \hat{n} \cdot \vec{v}_1 + \right. \\ & 8 \hat{n} \times \vec{S}_1 \cdot \vec{v}_1 \hat{n} \cdot \vec{v}_2 \hat{n} \cdot \vec{v}_1 + 3 \hat{n} \times \vec{S}_1 \cdot \vec{v}_2 \hat{n} \cdot \vec{v}_2 \hat{n} \cdot \vec{v}_1 - 4 \hat{n} \times \vec{S}_1 \cdot \vec{v}_1 (\hat{n} \cdot \vec{v}_2)^2 + \frac{11}{5} \vec{S}_1 \times \vec{v}_1 \cdot \vec{v}_2 \hat{n} \cdot \vec{v}_2 + \\ & \left. \left. \frac{2}{5} \hat{n} \times \vec{S}_1 \cdot \vec{v}_2 \vec{v}_1 \cdot \vec{v}_1 - \frac{8}{5} \hat{n} \times \vec{S}_1 \cdot \vec{v}_1 \vec{v}_1 \cdot \vec{v}_2 - \frac{3}{5} \hat{n} \times \vec{S}_1 \cdot \vec{v}_2 \vec{v}_1 \cdot \vec{v}_2 + \frac{4}{5} \hat{n} \times \vec{S}_1 \cdot \vec{v}_1 \vec{v}_2 \cdot \vec{v}_2 \right) \right) m_2^3 \Bigg\} \end{aligned}$$

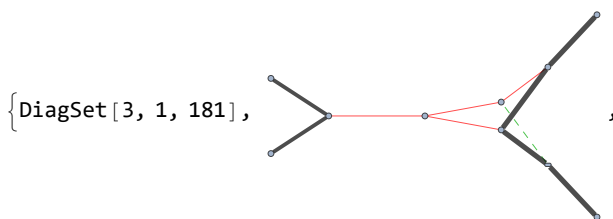

$$\begin{aligned} & \frac{1}{r^3} m_1^2 m_2 \left( -\frac{1}{5} \log \left( \frac{r}{R_0} \right) \vec{S}_1 \times \vec{v}_1 \cdot \vec{a}_1 - \frac{1}{25} \vec{S}_1 \times \vec{v}_1 \cdot \vec{a}_1 + \frac{7}{25} \hat{n} \times \vec{S}_1 \cdot \vec{v}_1 \hat{n} \cdot \vec{v}_1 + \frac{7}{25} \hat{n} \times \vec{S}_1 \cdot \vec{a}_1 \hat{n} \cdot \vec{v}_1 - \hat{n} \times \vec{S}_1 \cdot \vec{v}_1 \hat{n} \cdot \vec{v}_2 - \right. \\ & \hat{n} \times \vec{S}_1 \cdot \vec{a}_1 \hat{n} \cdot \vec{v}_2 - \vec{S}_1 \times \vec{v}_1 \cdot \vec{v}_2 \log \left( \frac{r}{R_0} \right) - \vec{S}_1 \times \vec{a}_1 \cdot \vec{v}_2 \log \left( \frac{r}{R_0} \right) - \frac{3}{5} \hat{n} \times \vec{S}_1 \cdot \vec{v}_1 \hat{n} \cdot \vec{v}_1 \log \left( \frac{r}{R_0} \right) - \\ & \frac{3}{5} \hat{n} \times \vec{S}_1 \cdot \vec{a}_1 \hat{n} \cdot \vec{v}_1 \log \left( \frac{r}{R_0} \right) + 3 \hat{n} \times \vec{S}_1 \cdot \vec{v}_1 \hat{n} \cdot \vec{v}_2 \log \left( \frac{r}{R_0} \right) + 3 \hat{n} \times \vec{S}_1 \cdot \vec{a}_1 \hat{n} \cdot \vec{v}_2 \log \left( \frac{r}{R_0} \right) + \frac{1}{\epsilon_d} \left( \frac{1}{3} \vec{S}_1 \times \vec{v}_1 \cdot \vec{v}_2 + \right. \\ & \frac{1}{3} \vec{S}_1 \times \vec{a}_1 \cdot \vec{v}_2 + \frac{1}{15} \vec{S}_1 \times \vec{v}_1 \cdot \vec{a}_1 + \frac{1}{5} \hat{n} \times \vec{S}_1 \cdot \vec{v}_1 \hat{n} \cdot \vec{v}_1 + \frac{1}{5} \hat{n} \times \vec{S}_1 \cdot \vec{a}_1 \hat{n} \cdot \vec{v}_1 - \hat{n} \times \vec{S}_1 \cdot \vec{v}_1 \hat{n} \cdot \vec{v}_2 - \hat{n} \times \vec{S}_1 \cdot \vec{a}_1 \hat{n} \cdot \vec{v}_2 \Bigg) G^3 + \\ & \frac{1}{r^4} m_1^2 m_2 \left( -\frac{58}{49} \hat{n} \times \vec{S}_1 \cdot \vec{v}_1 (\hat{n} \cdot \vec{v}_1)^2 + \frac{12}{7} \hat{n} \times \vec{S}_1 \cdot \vec{v}_1 \log \left( \frac{r}{R_0} \right) (\hat{n} \cdot \vec{v}_1)^2 - \vec{S}_1 \times \vec{v}_1 \cdot \vec{v}_2 \hat{n} \cdot \vec{v}_1 + \right. \end{aligned}$$

$$8 \hat{n} \times \vec{S}_1 \cdot \vec{v}_1 \hat{n} \cdot \vec{v}_2 \hat{n} \cdot \vec{v}_1 + 3 \vec{S}_1 \times \vec{v}_1 \cdot \vec{v}_2 \log\left(\frac{r}{R_\theta}\right) \hat{n} \cdot \vec{v}_1 - 15 \hat{n} \times \vec{S}_1 \cdot \vec{v}_1 \hat{n} \cdot \vec{v}_2 \log\left(\frac{r}{R_\theta}\right) \hat{n} \cdot \vec{v}_1 +$$

$$\frac{66 \hat{n} \times \vec{S}_1 \cdot \vec{v}_1 \vec{v}_1 \cdot \vec{v}_1}{1225} - \hat{n} \times \vec{S}_1 \cdot \vec{v}_1 \vec{v}_1 \cdot \vec{v}_2 - \frac{12}{35} \hat{n} \times \vec{S}_1 \cdot \vec{v}_1 \vec{v}_1 \cdot \vec{v}_1 \log\left(\frac{r}{R_\theta}\right) + 3 \hat{n} \times \vec{S}_1 \cdot \vec{v}_1 \vec{v}_1 \cdot \vec{v}_2 \log\left(\frac{r}{R_\theta}\right) + \frac{1}{\epsilon_d}$$

$$\left( -\frac{4}{7} \hat{n} \times \vec{S}_1 \cdot \vec{v}_1 (\hat{n} \cdot \vec{v}_1)^2 - \vec{S}_1 \times \vec{v}_1 \cdot \vec{v}_2 \hat{n} \cdot \vec{v}_1 + 5 \hat{n} \times \vec{S}_1 \cdot \vec{v}_1 \hat{n} \cdot \vec{v}_2 \hat{n} \cdot \vec{v}_1 + \frac{4}{35} \hat{n} \times \vec{S}_1 \cdot \vec{v}_1 \vec{v}_1 \cdot \vec{v}_1 - \hat{n} \times \vec{S}_1 \cdot \vec{v}_1 \vec{v}_1 \cdot \vec{v}_2 \right) G^3 \}$$

{DiagSet[3, 1, 182],

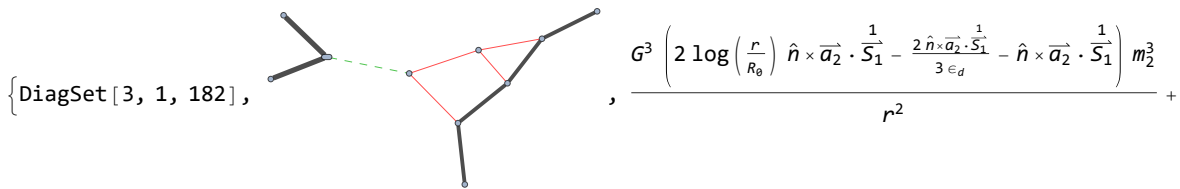

,  $\frac{G^3 \left( 2 \log\left(\frac{r}{R_\theta}\right) \hat{n} \times \vec{a}_2 \cdot \vec{S}_1 - \frac{2 \hat{n} \times \vec{a}_2 \cdot \vec{S}_1}{3 \epsilon_d} - \hat{n} \times \vec{a}_2 \cdot \vec{S}_1 \right) m_2^2}{r^2} +$

$$\frac{1}{r^3} G^3 \left( 2 \log\left(\frac{r}{R_\theta}\right) \vec{a}_2 \times \vec{S}_1 \cdot \vec{v}_1 - \vec{a}_2 \times \vec{S}_1 \cdot \vec{v}_1 + 2 \vec{a}_2 \times \vec{S}_1 \cdot \vec{v}_2 - \frac{108}{25} \hat{n} \times \vec{S}_1 \cdot \vec{v}_2 \hat{n} \cdot \vec{a}_2 + 5 \hat{n} \times \vec{a}_2 \cdot \vec{S}_1 \hat{n} \cdot \vec{v}_1 + \right.$$

$$\frac{107}{25} \hat{n} \times \vec{S}_1 \cdot \vec{v}_2 \hat{n} \cdot \vec{v}_2 - \frac{142}{25} \hat{n} \times \vec{a}_2 \cdot \vec{S}_1 \hat{n} \cdot \vec{v}_2 - 4 \vec{a}_2 \times \vec{S}_1 \cdot \vec{v}_2 \log\left(\frac{r}{R_\theta}\right) + \frac{27}{5} \hat{n} \times \vec{S}_1 \cdot \vec{v}_2 \hat{n} \cdot \vec{a}_2 \log\left(\frac{r}{R_\theta}\right) -$$

$$6 \hat{n} \times \vec{a}_2 \cdot \vec{S}_1 \hat{n} \cdot \vec{v}_1 \log\left(\frac{r}{R_\theta}\right) - \frac{18}{5} \hat{n} \times \vec{S}_1 \cdot \vec{v}_2 \hat{n} \cdot \vec{v}_2 \log\left(\frac{r}{R_\theta}\right) + \frac{33}{5} \hat{n} \times \vec{a}_2 \cdot \vec{S}_1 \hat{n} \cdot \vec{v}_2 \log\left(\frac{r}{R_\theta}\right) + \frac{1}{\epsilon_d}$$

$$\left( -\frac{2}{3} \vec{a}_2 \times \vec{S}_1 \cdot \vec{v}_1 + \frac{4}{3} \vec{a}_2 \times \vec{S}_1 \cdot \vec{v}_2 - \frac{9}{5} \hat{n} \times \vec{S}_1 \cdot \vec{v}_2 \hat{n} \cdot \vec{a}_2 + 2 \hat{n} \times \vec{a}_2 \cdot \vec{S}_1 \hat{n} \cdot \vec{v}_1 + \frac{6}{5} \hat{n} \times \vec{S}_1 \cdot \vec{v}_2 \hat{n} \cdot \vec{v}_2 - \frac{11}{5} \hat{n} \times \vec{a}_2 \cdot \vec{S}_1 \hat{n} \cdot \vec{v}_2 \right) \Bigg)$$

$$m_2^3 + \frac{1}{r^4} G^3 \left( 7 \hat{n} \times \vec{S}_1 \cdot \vec{v}_2 (\hat{n} \cdot \vec{v}_2)^2 - 3 \hat{n} \times \vec{S}_1 \cdot \vec{v}_2 \log\left(\frac{r}{R_\theta}\right) (\hat{n} \cdot \vec{v}_2)^2 - \frac{107}{25} \vec{S}_1 \times \vec{v}_1 \cdot \vec{v}_2 \hat{n} \cdot \vec{v}_2 - \right.$$

$$25 \hat{n} \times \vec{S}_1 \cdot \vec{v}_2 \hat{n} \cdot \vec{v}_1 \hat{n} \cdot \vec{v}_2 + \frac{18}{5} \vec{S}_1 \times \vec{v}_1 \cdot \vec{v}_2 \log\left(\frac{r}{R_\theta}\right) \hat{n} \cdot \vec{v}_2 + 18 \hat{n} \times \vec{S}_1 \cdot \vec{v}_2 \hat{n} \cdot \vec{v}_1 \log\left(\frac{r}{R_\theta}\right) \hat{n} \cdot \vec{v}_2 +$$

$$\frac{107}{25} \hat{n} \times \vec{S}_1 \cdot \vec{v}_2 \vec{v}_1 \cdot \vec{v}_2 + \frac{8}{25} \hat{n} \times \vec{S}_1 \cdot \vec{v}_2 \vec{v}_2 \cdot \vec{v}_2 - \frac{18}{5} \hat{n} \times \vec{S}_1 \cdot \vec{v}_2 \vec{v}_1 \cdot \vec{v}_2 \log\left(\frac{r}{R_\theta}\right) + \frac{3}{5} \hat{n} \times \vec{S}_1 \cdot \vec{v}_2 \vec{v}_2 \cdot \vec{v}_2 \log\left(\frac{r}{R_\theta}\right) + \frac{1}{\epsilon_d}$$

$$\left. \left( \hat{n} \times \vec{S}_1 \cdot \vec{v}_2 (\hat{n} \cdot \vec{v}_2)^2 - \frac{6}{5} \vec{S}_1 \times \vec{v}_1 \cdot \vec{v}_2 \hat{n} \cdot \vec{v}_2 - 6 \hat{n} \times \vec{S}_1 \cdot \vec{v}_2 \hat{n} \cdot \vec{v}_1 \hat{n} \cdot \vec{v}_2 + \frac{6}{5} \hat{n} \times \vec{S}_1 \cdot \vec{v}_2 \vec{v}_1 \cdot \vec{v}_2 - \frac{1}{5} \hat{n} \times \vec{S}_1 \cdot \vec{v}_2 \vec{v}_2 \cdot \vec{v}_2 \right) \right) m_2^3 \}$$

{DiagSet[3, 1, 183],

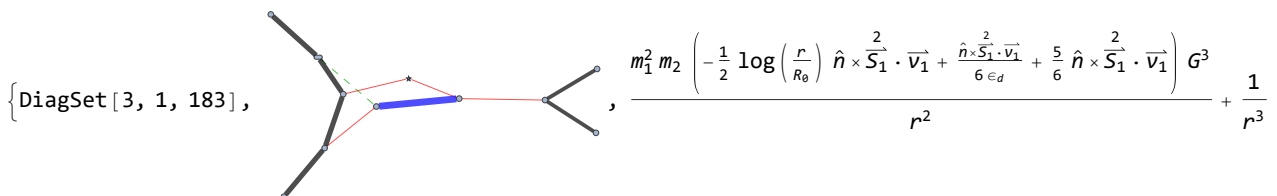

,  $\frac{m_1^2 m_2 \left( -\frac{1}{2} \log\left(\frac{r}{R_\theta}\right) \hat{n} \times \vec{S}_1 \cdot \vec{v}_1 + \frac{\hat{n} \times \vec{S}_1 \cdot \vec{v}_1}{6 \epsilon_d} + \frac{5}{6} \hat{n} \times \vec{S}_1 \cdot \vec{v}_1 \right) G^3}{r^2} + \frac{1}{r^3}$

$$m_1^2 m_2 \left( \frac{1}{2} \log\left(\frac{r}{R_\theta}\right) \vec{S}_1 \times \vec{v}_1 \cdot \vec{v}_2 - \frac{5}{6} \vec{S}_1 \times \vec{v}_1 \cdot \vec{v}_2 - \frac{1}{2} \vec{S}_1 \times \vec{v}_1 \cdot \vec{a}_1 - \frac{34}{25} \hat{n} \times \vec{S}_1 \cdot \vec{v}_1 \hat{n} \cdot \vec{v}_1 - \hat{n} \times \vec{S}_1 \cdot \vec{a}_1 \hat{n} \cdot \vec{v}_1 + 3 \hat{n} \times \vec{S}_1 \cdot \vec{v}_1 \hat{n} \cdot \vec{v}_2 + \right.$$

$$\frac{1}{2} \vec{S}_1 \times \vec{v}_1 \cdot \vec{a}_1 \log\left(\frac{r}{R_\theta}\right) + \frac{6}{5} \hat{n} \times \vec{S}_1 \cdot \vec{v}_1 \hat{n} \cdot \vec{v}_1 \log\left(\frac{r}{R_\theta}\right) + \frac{3}{2} \hat{n} \times \vec{S}_1 \cdot \vec{a}_1 \hat{n} \cdot \vec{v}_1 \log\left(\frac{r}{R_\theta}\right) - \frac{3}{2} \hat{n} \times \vec{S}_1 \cdot \vec{v}_1 \hat{n} \cdot \vec{v}_2 \log\left(\frac{r}{R_\theta}\right) +$$

$$\frac{1}{\epsilon_d} \left( -\frac{1}{6} \vec{S}_1 \times \vec{v}_1 \cdot \vec{v}_2 - \frac{1}{6} \vec{S}_1 \times \vec{v}_1 \cdot \vec{a}_1 - \frac{2}{5} \hat{n} \times \vec{S}_1 \cdot \vec{v}_1 \hat{n} \cdot \vec{v}_1 - \frac{1}{2} \hat{n} \times \vec{S}_1 \cdot \vec{a}_1 \hat{n} \cdot \vec{v}_1 + \frac{1}{2} \hat{n} \times \vec{S}_1 \cdot \vec{v}_1 \hat{n} \cdot \vec{v}_2 \right) \Bigg) G^3 + \frac{1}{r^4}$$

$$m_1^2 m_2 \left( 3 \hat{n} \times \vec{S}_1 \cdot \vec{v}_1 (\hat{n} \cdot \vec{v}_1)^2 - 3 \hat{n} \times \vec{S}_1 \cdot \vec{v}_1 \log\left(\frac{r}{R_\theta}\right) (\hat{n} \cdot \vec{v}_1)^2 + \vec{S}_1 \times \vec{v}_1 \cdot \vec{v}_2 \hat{n} \cdot \vec{v}_1 - \frac{13}{2} \hat{n} \times \vec{S}_1 \cdot \vec{v}_1 \hat{n} \cdot \vec{v}_2 \hat{n} \cdot \vec{v}_1 - \right.$$

$$\frac{3}{2} \vec{S}_1 \times \vec{v}_1 \cdot \vec{v}_2 \log\left(\frac{r}{R_\theta}\right) \hat{n} \cdot \vec{v}_1 + \frac{15}{2} \hat{n} \times \vec{S}_1 \cdot \vec{v}_1 \hat{n} \cdot \vec{v}_2 \log\left(\frac{r}{R_\theta}\right) \hat{n} \cdot \vec{v}_1 - \frac{2}{25} \hat{n} \times \vec{S}_1 \cdot \vec{v}_1 \vec{v}_1 \cdot \vec{v}_1 +$$

$$\hat{n} \times \vec{S}_1 \cdot \vec{v}_1 \vec{v}_1 \cdot \vec{v}_2 + \frac{3}{5} \hat{n} \times \vec{S}_1 \cdot \vec{v}_1 \vec{v}_1 \cdot \vec{v}_1 \log\left(\frac{r}{R_\theta}\right) - \frac{3}{2} \hat{n} \times \vec{S}_1 \cdot \vec{v}_1 \vec{v}_1 \cdot \vec{v}_2 \log\left(\frac{r}{R_\theta}\right) + \frac{1}{\epsilon_d} \left( \hat{n} \times \vec{S}_1 \cdot \vec{v}_1 (\hat{n} \cdot \vec{v}_1)^2 + \right.$$

$$\left. \frac{1}{2} \vec{S}_1 \times \vec{v}_1 \cdot \vec{v}_2 \hat{n} \cdot \vec{v}_1 - \frac{5}{2} \hat{n} \times \vec{S}_1 \cdot \vec{v}_1 \hat{n} \cdot \vec{v}_2 \hat{n} \cdot \vec{v}_1 - \frac{1}{5} \hat{n} \times \vec{S}_1 \cdot \vec{v}_1 \vec{v}_1 \cdot \vec{v}_1 + \frac{1}{2} \hat{n} \times \vec{S}_1 \cdot \vec{v}_1 \vec{v}_1 \cdot \vec{v}_2 \right) \Bigg) G^3 \}$$

{DiagSet[3, 1, 184],

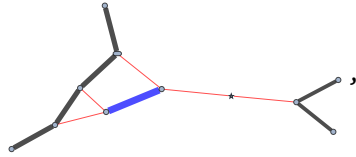

$$\frac{1}{r^3} G^3 m_1^2 m_2 \left( \frac{-\frac{3}{5} \hat{n} \cdot \vec{v}_2 \hat{n} \times \vec{S}_1 \cdot \vec{a}_1 + \frac{1}{5} \vec{S}_1 \times \vec{a}_1 \cdot \vec{v}_2 - \frac{3}{5} \hat{n} \cdot \vec{v}_2 \hat{n} \times \vec{S}_1 \cdot \vec{v}_1 + \frac{1}{5} \vec{S}_1 \times \vec{v}_1 \cdot \vec{v}_2}{\epsilon_d} + \right.$$

$$\frac{9}{5} \log\left(\frac{r}{R_\theta}\right) \hat{n} \cdot \vec{v}_2 \hat{n} \times \vec{S}_1 \cdot \vec{a}_1 - \frac{97}{50} \hat{n} \cdot \vec{v}_2 \hat{n} \times \vec{S}_1 \cdot \vec{a}_1 - \frac{3}{5} \log\left(\frac{r}{R_\theta}\right) \vec{S}_1 \times \vec{a}_1 \cdot \vec{v}_2 + \frac{67}{150} \vec{S}_1 \times \vec{a}_1 \cdot \vec{v}_2 +$$

$$\left. \frac{9}{5} \log\left(\frac{r}{R_\theta}\right) \hat{n} \cdot \vec{v}_2 \hat{n} \times \vec{S}_1 \cdot \vec{v}_1 - \frac{97}{50} \hat{n} \cdot \vec{v}_2 \hat{n} \times \vec{S}_1 \cdot \vec{v}_1 - \frac{3}{5} \log\left(\frac{r}{R_\theta}\right) \vec{S}_1 \times \vec{v}_1 \cdot \vec{v}_2 + \frac{67}{150} \vec{S}_1 \times \vec{v}_1 \cdot \vec{v}_2 \right) +$$

$$\frac{1}{r^4} G^3 m_1^2 m_2 \left( \frac{-\frac{3}{5} \hat{n} \cdot \vec{v}_1 \vec{S}_1 \times \vec{v}_1 \cdot \vec{v}_2 + 3 \hat{n} \cdot \vec{v}_2 \hat{n} \cdot \vec{v}_1 \hat{n} \times \vec{S}_1 \cdot \vec{v}_1 - \frac{3}{5} \vec{v}_1 \cdot \vec{v}_2 \hat{n} \times \vec{S}_1 \cdot \vec{v}_1}{\epsilon_d} + \right.$$

$$\frac{9}{5} \log\left(\frac{r}{R_\theta}\right) \hat{n} \cdot \vec{v}_1 \vec{S}_1 \times \vec{v}_1 \cdot \vec{v}_2 - 9 \log\left(\frac{r}{R_\theta}\right) \hat{n} \cdot \vec{v}_2 \hat{n} \cdot \vec{v}_1 \hat{n} \times \vec{S}_1 \cdot \vec{v}_1 + \frac{9}{5} \log\left(\frac{r}{R_\theta}\right) \vec{v}_1 \cdot \vec{v}_2 \hat{n} \times \vec{S}_1 \cdot \vec{v}_1 -$$

$$\left. \frac{97}{50} \hat{n} \cdot \vec{v}_1 \vec{S}_1 \times \vec{v}_1 \cdot \vec{v}_2 + \frac{23}{2} \hat{n} \cdot \vec{v}_2 \hat{n} \cdot \vec{v}_1 \hat{n} \times \vec{S}_1 \cdot \vec{v}_1 - \frac{97}{50} \vec{v}_1 \cdot \vec{v}_2 \hat{n} \times \vec{S}_1 \cdot \vec{v}_1 \right\}$$

{DiagSet[3, 1, 185],

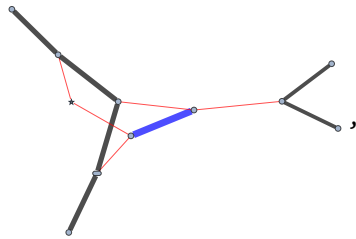

$$\frac{1}{r^3} G^3 m_1^2 m_2 \left( \frac{\frac{3}{5} \hat{n} \cdot \vec{v}_1 \hat{n} \times \vec{S}_1 \cdot \vec{a}_1 + \frac{1}{5} \vec{S}_1 \times \vec{v}_1 \cdot \vec{a}_1 + \frac{3}{5} \hat{n} \cdot \vec{v}_1 \hat{n} \times \vec{S}_1 \cdot \vec{v}_1}{\epsilon_d} - \frac{9}{5} \log\left(\frac{r}{R_\theta}\right) \hat{n} \cdot \vec{v}_1 \hat{n} \times \vec{S}_1 \cdot \vec{a}_1 + \frac{51}{25} \hat{n} \cdot \vec{v}_1 \hat{n} \times \vec{S}_1 \cdot \vec{a}_1 - \right.$$

$$\left. \frac{3}{5} \log\left(\frac{r}{R_\theta}\right) \vec{S}_1 \times \vec{v}_1 \cdot \vec{a}_1 + \frac{46}{75} \vec{S}_1 \times \vec{v}_1 \cdot \vec{a}_1 - \frac{9}{5} \log\left(\frac{r}{R_\theta}\right) \hat{n} \cdot \vec{v}_1 \hat{n} \times \vec{S}_1 \cdot \vec{v}_1 + \frac{51}{25} \hat{n} \cdot \vec{v}_1 \hat{n} \times \vec{S}_1 \cdot \vec{v}_1 \right) + \frac{1}{r^4}$$

$$G^3 m_1^2 m_2 \left( \frac{1}{\epsilon_d} \left( -\frac{19}{7} (\hat{n} \cdot \vec{v}_1)^2 \hat{n} \times \vec{S}_1 \cdot \vec{v}_1 - \frac{3}{5} \hat{n} \cdot \vec{v}_1 \vec{S}_1 \times \vec{v}_1 \cdot \vec{v}_2 + 3 \hat{n} \cdot \vec{v}_2 \hat{n} \cdot \vec{v}_1 \hat{n} \times \vec{S}_1 \cdot \vec{v}_1 + \frac{19}{35} \vec{v}_1 \cdot \vec{v}_1 \hat{n} \times \vec{S}_1 \cdot \vec{v}_1 - \right. \right.$$

$$\frac{3}{5} \vec{v}_1 \cdot \vec{v}_2 \hat{n} \times \vec{S}_1 \cdot \vec{v}_1 \left. \right) + \frac{57}{7} \log\left(\frac{r}{R_\theta}\right) (\hat{n} \cdot \vec{v}_1)^2 \hat{n} \times \vec{S}_1 \cdot \vec{v}_1 + \frac{9}{5} \log\left(\frac{r}{R_\theta}\right) \hat{n} \cdot \vec{v}_1 \vec{S}_1 \times \vec{v}_1 \cdot \vec{v}_2 - 9 \log\left(\frac{r}{R_\theta}\right) \hat{n} \cdot \vec{v}_2$$

$$\hat{n} \cdot \vec{v}_1 \hat{n} \times \vec{S}_1 \cdot \vec{v}_1 - \frac{57}{35} \log\left(\frac{r}{R_\theta}\right) \vec{v}_1 \cdot \vec{v}_1 \hat{n} \times \vec{S}_1 \cdot \vec{v}_1 + \frac{9}{5} \log\left(\frac{r}{R_\theta}\right) \vec{v}_1 \cdot \vec{v}_2 \hat{n} \times \vec{S}_1 \cdot \vec{v}_1 - \frac{510}{49} (\hat{n} \cdot \vec{v}_1)^2 \hat{n} \times \vec{S}_1 \cdot \vec{v}_1 -$$

$$\left. \frac{51}{25} \hat{n} \cdot \vec{v}_1 \vec{S}_1 \times \vec{v}_1 \cdot \vec{v}_2 + 12 \hat{n} \cdot \vec{v}_2 \hat{n} \cdot \vec{v}_1 \hat{n} \times \vec{S}_1 \cdot \vec{v}_1 + \frac{2711 \vec{v}_1 \cdot \vec{v}_1 \hat{n} \times \vec{S}_1 \cdot \vec{v}_1}{1225} - \frac{51}{25} \vec{v}_1 \cdot \vec{v}_2 \hat{n} \times \vec{S}_1 \cdot \vec{v}_1 \right\}$$



{DiagSet[3, 1, 186],

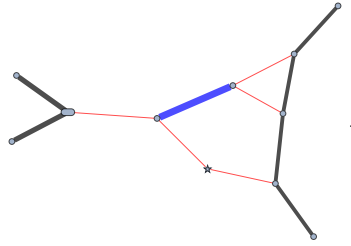

$$\frac{G^3 m_2^3 \left( -\hat{n} \cdot \vec{v}_2 \hat{n} \times \vec{a}_1 \cdot \vec{S}_1 + \frac{1}{3} \vec{a}_1 \times \vec{S}_1 \cdot \vec{v}_2 + \hat{n} \cdot \vec{v}_2 \hat{n} \times \vec{S}_1 \cdot \vec{v}_1 - \frac{1}{3} \vec{S}_1 \times \vec{v}_1 \cdot \vec{v}_2 \right)}{r^3} + \frac{1}{r^4}$$

$$G^3 m_2^3 \left( \frac{\left( \hat{n} \cdot \vec{v}_2 \right)^2 \left( -\left( \hat{n} \times \vec{S}_1 \cdot \vec{v}_1 \right) \right) + \frac{2}{5} \hat{n} \cdot \vec{v}_2 \vec{S}_1 \times \vec{v}_1 \cdot \vec{v}_2 + \frac{1}{5} \vec{v}_2 \cdot \vec{v}_2 \hat{n} \times \vec{S}_1 \cdot \vec{v}_1}{\epsilon_d} + 3 \log \left( \frac{r}{R_\theta} \right) \left( \hat{n} \cdot \vec{v}_2 \right)^2 \hat{n} \times \vec{S}_1 \cdot \vec{v}_1 - \right.$$

$$\frac{6}{5} \log \left( \frac{r}{R_\theta} \right) \hat{n} \cdot \vec{v}_2 \vec{S}_1 \times \vec{v}_1 \cdot \vec{v}_2 - \frac{3}{5} \log \left( \frac{r}{R_\theta} \right) \vec{v}_2 \cdot \vec{v}_2 \hat{n} \times \vec{S}_1 \cdot \vec{v}_1 - 2 \left( \hat{n} \cdot \vec{v}_2 \right)^2 \hat{n} \times \vec{S}_1 \cdot \vec{v}_1 + \frac{14}{25} \hat{n} \cdot \vec{v}_2 \vec{S}_1 \times \vec{v}_1 \cdot \vec{v}_2 -$$

$$\left. 5 \hat{n} \cdot \vec{v}_1 \hat{n} \cdot \vec{v}_2 \hat{n} \times \vec{S}_1 \cdot \vec{v}_1 + \hat{n} \cdot \vec{v}_1 \vec{S}_1 \times \vec{v}_1 \cdot \vec{v}_2 + \vec{v}_1 \cdot \vec{v}_2 \hat{n} \times \vec{S}_1 \cdot \vec{v}_1 + \frac{27}{25} \vec{v}_2 \cdot \vec{v}_2 \hat{n} \times \vec{S}_1 \cdot \vec{v}_1 \right\}$$

{DiagSet[3, 1, 187],

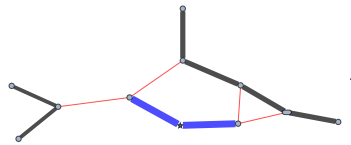

$$\frac{1}{r^3} G^3 m_1^2 m_2 \left( \frac{\frac{1}{5} \hat{n} \cdot \vec{v}_1 \hat{n} \times \vec{S}_1 \cdot \vec{a}_1 + \frac{1}{15} \vec{S}_1 \times \vec{v}_1 \cdot \vec{a}_1 + \frac{1}{5} \hat{n} \cdot \vec{v}_1 \hat{n} \times \vec{S}_1 \cdot \vec{v}_1}{\epsilon_d} - \frac{3}{5} \log \left( \frac{r}{R_\theta} \right) \hat{n} \cdot \vec{v}_1 \hat{n} \times \vec{S}_1 \cdot \vec{a}_1 + \right.$$

$$\frac{16}{75} \hat{n} \cdot \vec{v}_1 \hat{n} \times \vec{S}_1 \cdot \vec{a}_1 + \frac{2}{3} \hat{n} \cdot \vec{v}_2 \hat{n} \times \vec{S}_1 \cdot \vec{a}_1 - \frac{1}{5} \log \left( \frac{r}{R_\theta} \right) \vec{S}_1 \times \vec{v}_1 \cdot \vec{a}_1 - \frac{2}{9} \vec{S}_1 \times \vec{a}_1 \cdot \vec{v}_2 + \frac{61}{225} \vec{S}_1 \times \vec{v}_1 \cdot \vec{a}_1 -$$

$$\left. \frac{3}{5} \log \left( \frac{r}{R_\theta} \right) \hat{n} \cdot \vec{v}_1 \hat{n} \times \vec{S}_1 \cdot \vec{v}_1 + \frac{16}{75} \hat{n} \cdot \vec{v}_1 \hat{n} \times \vec{S}_1 \cdot \vec{v}_1 + \frac{2}{3} \hat{n} \cdot \vec{v}_2 \hat{n} \times \vec{S}_1 \cdot \vec{v}_1 - \frac{2}{9} \frac{1}{\vec{S}_1 \times \vec{v}_1 \cdot \vec{v}_2} \right) + \frac{1}{r^4} G^3 m_1^2 m_2$$

$$\left( \frac{1}{\epsilon_d} \left( \frac{1}{7} \left( \hat{n} \cdot \vec{v}_1 \right)^2 \hat{n} \times \vec{S}_1 \cdot \vec{v}_1 + \frac{1}{5} \hat{n} \cdot \vec{v}_1 \vec{S}_1 \times \vec{v}_1 \cdot \vec{v}_2 - \hat{n} \cdot \vec{v}_2 \hat{n} \cdot \vec{v}_1 \hat{n} \times \vec{S}_1 \cdot \vec{v}_1 - \frac{1}{35} \vec{v}_1 \cdot \vec{v}_1 \hat{n} \times \vec{S}_1 \cdot \vec{v}_1 + \frac{1}{5} \vec{v}_1 \cdot \vec{v}_2 \hat{n} \times \vec{S}_1 \cdot \vec{v}_1 \right) - \right.$$

$$\frac{3}{7} \log \left( \frac{r}{R_\theta} \right) \left( \hat{n} \cdot \vec{v}_1 \right)^2 \hat{n} \times \vec{S}_1 \cdot \vec{v}_1 - \frac{3}{5} \log \left( \frac{r}{R_\theta} \right) \hat{n} \cdot \vec{v}_1 \vec{S}_1 \times \vec{v}_1 \cdot \vec{v}_2 + 3 \log \left( \frac{r}{R_\theta} \right) \hat{n} \cdot \vec{v}_2 \hat{n} \cdot \vec{v}_1 \hat{n} \times \vec{S}_1 \cdot \vec{v}_1 +$$

$$\frac{3}{35} \log \left( \frac{r}{R_\theta} \right) \vec{v}_1 \cdot \vec{v}_1 \hat{n} \times \vec{S}_1 \cdot \vec{v}_1 - \frac{3}{5} \log \left( \frac{r}{R_\theta} \right) \vec{v}_1 \cdot \vec{v}_2 \hat{n} \times \vec{S}_1 \cdot \vec{v}_1 + \frac{89}{147} \left( \hat{n} \cdot \vec{v}_1 \right)^2 \hat{n} \times \vec{S}_1 \cdot \vec{v}_1 +$$

$$\left. \frac{22}{25} \hat{n} \cdot \vec{v}_1 \vec{S}_1 \times \vec{v}_1 \cdot \vec{v}_2 - 5 \hat{n} \cdot \vec{v}_2 \hat{n} \cdot \vec{v}_1 \hat{n} \times \vec{S}_1 \cdot \vec{v}_1 + \frac{458 \vec{v}_1 \cdot \vec{v}_1 \hat{n} \times \vec{S}_1 \cdot \vec{v}_1}{3675} + \frac{22}{25} \vec{v}_1 \cdot \vec{v}_2 \hat{n} \times \vec{S}_1 \cdot \vec{v}_1 \right\}$$

{DiagSet[3, 1, 188],

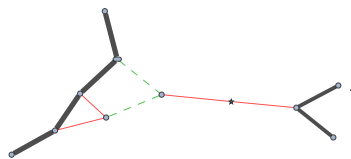

$$\begin{aligned}
& \frac{1}{r^3} G^3 m_1^2 m_2 \left( \frac{\frac{1}{10} \hat{n} \cdot \vec{v}_2 \hat{n} \times \vec{S}_1 \cdot \vec{a}_1 - \frac{1}{30} \vec{S}_1 \times \vec{a}_1 \cdot \vec{v}_2 + \frac{1}{10} \hat{n} \cdot \vec{v}_2 \hat{n} \times \vec{S}_1 \cdot \vec{v}_1 - \frac{1}{30} \vec{S}_1 \times \vec{v}_1 \cdot \vec{v}_2}{\epsilon_d} - \right. \\
& \frac{3}{10} \log\left(\frac{r}{R_0}\right) \hat{n} \cdot \vec{v}_2 \hat{n} \times \vec{S}_1 \cdot \vec{a}_1 + \frac{7}{50} \hat{n} \cdot \vec{v}_2 \hat{n} \times \vec{S}_1 \cdot \vec{a}_1 + \frac{1}{10} \log\left(\frac{r}{R_0}\right) \vec{S}_1 \times \vec{a}_1 \cdot \vec{v}_2 - \frac{1}{75} \vec{S}_1 \times \vec{a}_1 \cdot \vec{v}_2 - \\
& \left. \frac{3}{10} \log\left(\frac{r}{R_0}\right) \hat{n} \cdot \vec{v}_2 \hat{n} \times \vec{S}_1 \cdot \vec{v}_1 + \frac{7}{50} \hat{n} \cdot \vec{v}_2 \hat{n} \times \vec{S}_1 \cdot \vec{v}_1 + \frac{1}{10} \log\left(\frac{r}{R_0}\right) \vec{S}_1 \times \vec{v}_1 \cdot \vec{v}_2 - \frac{1}{75} \vec{S}_1 \times \vec{v}_1 \cdot \vec{v}_2 \right) + \\
& \frac{1}{r^4} G^3 m_1^2 m_2 \left( \frac{\frac{1}{10} \hat{n} \cdot \vec{v}_1 \vec{S}_1 \times \vec{v}_1 \cdot \vec{v}_2 - \frac{1}{2} \hat{n} \cdot \vec{v}_2 \hat{n} \cdot \vec{v}_1 \hat{n} \times \vec{S}_1 \cdot \vec{v}_1 + \frac{1}{10} \vec{v}_1 \cdot \vec{v}_2 \hat{n} \times \vec{S}_1 \cdot \vec{v}_1}{\epsilon_d} - \right. \\
& \frac{3}{10} \log\left(\frac{r}{R_0}\right) \hat{n} \cdot \vec{v}_1 \vec{S}_1 \times \vec{v}_1 \cdot \vec{v}_2 + \frac{3}{2} \log\left(\frac{r}{R_0}\right) \hat{n} \cdot \vec{v}_2 \hat{n} \cdot \vec{v}_1 \hat{n} \times \vec{S}_1 \cdot \vec{v}_1 - \frac{3}{10} \log\left(\frac{r}{R_0}\right) \vec{v}_1 \cdot \vec{v}_2 \hat{n} \times \vec{S}_1 \cdot \vec{v}_1 + \\
& \left. \frac{7}{50} \hat{n} \cdot \vec{v}_1 \vec{S}_1 \times \vec{v}_1 \cdot \vec{v}_2 - \hat{n} \cdot \vec{v}_2 \hat{n} \cdot \vec{v}_1 \hat{n} \times \vec{S}_1 \cdot \vec{v}_1 + \frac{7}{50} \vec{v}_1 \cdot \vec{v}_2 \hat{n} \times \vec{S}_1 \cdot \vec{v}_1 \right) \Big\}
\end{aligned}$$

{DiagSet[3, 1, 189],

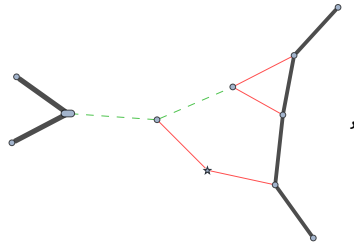

,

$$\begin{aligned}
& \frac{1}{r^3} G^3 m_2^3 \left( \frac{-\frac{1}{2} \hat{n} \cdot \vec{a}_2 \hat{n} \times \vec{S}_1 \cdot \vec{v}_2 - \frac{1}{2} \hat{n} \cdot \vec{v}_2 \hat{n} \times \vec{a}_2 \cdot \vec{S}_1 + \frac{1}{3} \vec{a}_2 \times \vec{S}_1 \cdot \vec{v}_2}{\epsilon_d} + \frac{3}{2} \log\left(\frac{r}{R_0}\right) \hat{n} \cdot \vec{a}_2 \hat{n} \times \vec{S}_1 \cdot \vec{v}_2 + \frac{3}{2} \log\left(\frac{r}{R_0}\right) \hat{n} \cdot \vec{v}_2 \right. \\
& \left. \hat{n} \times \vec{a}_2 \cdot \vec{S}_1 - \frac{1}{2} \hat{n} \cdot \vec{a}_2 \hat{n} \times \vec{S}_1 \cdot \vec{v}_2 - \frac{3}{2} \hat{n} \cdot \vec{v}_2 \hat{n} \times \vec{a}_2 \cdot \vec{S}_1 - \log\left(\frac{r}{R_0}\right) \vec{a}_2 \times \vec{S}_1 \cdot \vec{v}_2 + \frac{1}{3} \vec{a}_2 \times \vec{S}_1 \cdot \vec{v}_2 + \hat{n} \cdot \vec{v}_2 \hat{n} \times \vec{S}_1 \cdot \vec{v}_2 \right) + \\
& \left. \frac{1}{r^4} G^3 m_2^3 \left( 4 (\hat{n} \cdot \vec{v}_2)^2 \hat{n} \times \vec{S}_1 \cdot \vec{v}_2 - \hat{n} \cdot \vec{v}_2 \vec{S}_1 \times \vec{v}_1 \cdot \vec{v}_2 - 5 \hat{n} \cdot \vec{v}_1 \hat{n} \cdot \vec{v}_2 \hat{n} \times \vec{S}_1 \cdot \vec{v}_2 + \vec{v}_1 \cdot \vec{v}_2 \hat{n} \times \vec{S}_1 \cdot \vec{v}_2 \right) \right\}
\end{aligned}$$

{DiagSet[3, 1, 190],

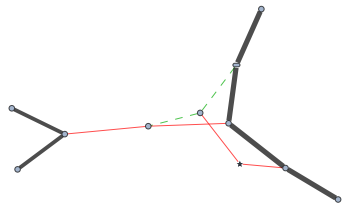

,

$$\begin{aligned}
& \frac{1}{r^3} m_1^2 m_2 \left( -\log\left(\frac{r}{R_0}\right) \vec{S}_1 \times \vec{v}_1 \cdot \vec{v}_2 + \frac{5}{6} \vec{S}_1 \times \vec{v}_1 \cdot \vec{v}_2 + \frac{1}{75} \vec{S}_1 \times \vec{v}_1 \cdot \vec{a}_1 + \frac{5}{6} \vec{S}_1 \times \vec{v}_1 \cdot \vec{a}_2 - \frac{28}{25} \hat{n} \times \vec{S}_1 \cdot \vec{v}_1 \hat{n} \cdot \vec{a}_1 - \right. \\
& \frac{7}{2} \hat{n} \times \vec{S}_1 \cdot \vec{v}_1 \hat{n} \cdot \vec{a}_2 - \frac{3}{2} \hat{n} \times \vec{S}_1 \cdot \vec{v}_1 \hat{n} \cdot \vec{v}_1 - \frac{19}{50} \hat{n} \times \vec{S}_1 \cdot \vec{a}_1 \hat{n} \cdot \vec{v}_1 - \frac{7}{2} \hat{n} \times \vec{S}_1 \cdot \vec{v}_1 \hat{n} \cdot \vec{v}_2 - \frac{1}{10} \vec{S}_1 \times \vec{v}_1 \cdot \vec{a}_1 \log\left(\frac{r}{R_0}\right) - \\
& \vec{S}_1 \times \vec{v}_1 \cdot \vec{a}_2 \log\left(\frac{r}{R_0}\right) + \frac{9}{10} \hat{n} \times \vec{S}_1 \cdot \vec{v}_1 \hat{n} \cdot \vec{a}_1 \log\left(\frac{r}{R_0}\right) + 3 \hat{n} \times \vec{S}_1 \cdot \vec{v}_1 \hat{n} \cdot \vec{a}_2 \log\left(\frac{r}{R_0}\right) + \frac{3}{2} \hat{n} \times \vec{S}_1 \cdot \vec{v}_1 \hat{n} \cdot \vec{v}_1 \log\left(\frac{r}{R_0}\right) + \\
& \frac{3}{5} \hat{n} \times \vec{S}_1 \cdot \vec{a}_1 \hat{n} \cdot \vec{v}_1 \log\left(\frac{r}{R_0}\right) + 3 \hat{n} \times \vec{S}_1 \cdot \vec{v}_1 \hat{n} \cdot \vec{v}_2 \log\left(\frac{r}{R_0}\right) + \frac{1}{\epsilon_d} \left( \frac{1}{3} \vec{S}_1 \times \vec{v}_1 \cdot \vec{v}_2 + \frac{1}{30} \vec{S}_1 \times \vec{v}_1 \cdot \vec{a}_1 + \frac{1}{3} \vec{S}_1 \times \vec{v}_1 \cdot \vec{a}_2 - \right. \\
& \left. \left. \frac{3}{10} \hat{n} \times \vec{S}_1 \cdot \vec{v}_1 \hat{n} \cdot \vec{a}_1 - \hat{n} \times \vec{S}_1 \cdot \vec{v}_1 \hat{n} \cdot \vec{a}_2 - \frac{1}{2} \hat{n} \times \vec{S}_1 \cdot \vec{v}_1 \hat{n} \cdot \vec{v}_1 - \frac{1}{5} \hat{n} \times \vec{S}_1 \cdot \vec{a}_1 \hat{n} \cdot \vec{v}_1 - \hat{n} \times \vec{S}_1 \cdot \vec{v}_1 \hat{n} \cdot \vec{v}_2 \right) \right) G^3 + \frac{1}{r^4}
\end{aligned}$$

$$m_1^2 m_2 \left( \frac{747}{98} \hat{n} \times \vec{S}_1 \cdot \vec{v}_1 (\hat{n} \cdot \vec{v}_1)^2 - \frac{93}{14} \hat{n} \times \vec{S}_1 \cdot \vec{v}_1 \log\left(\frac{r}{R_\theta}\right) (\hat{n} \cdot \vec{v}_1)^2 - \frac{28}{25} \vec{S}_1 \times \vec{v}_1 \cdot \vec{v}_2 \hat{n} \cdot \vec{v}_1 + \frac{13}{2} \hat{n} \times \vec{S}_1 \cdot \vec{v}_1 \hat{n} \cdot \vec{v}_2 \hat{n} \cdot \vec{v}_1 + \right. \\ \left. \frac{9}{10} \vec{S}_1 \times \vec{v}_1 \cdot \vec{v}_2 \log\left(\frac{r}{R_\theta}\right) \hat{n} \cdot \vec{v}_1 - \frac{9}{2} \hat{n} \times \vec{S}_1 \cdot \vec{v}_1 \hat{n} \cdot \vec{v}_2 \log\left(\frac{r}{R_\theta}\right) \hat{n} \cdot \vec{v}_1 - \frac{41}{2} \hat{n} \times \vec{S}_1 \cdot \vec{v}_1 (\hat{n} \cdot \vec{v}_2)^2 + 7 \vec{S}_1 \times \vec{v}_1 \cdot \vec{v}_2 \hat{n} \cdot \vec{v}_2 - \right. \\ \left. \frac{1612 \hat{n} \times \vec{S}_1 \cdot \vec{v}_1 \vec{v}_1 \cdot \vec{v}_1}{1225} - \frac{28}{25} \hat{n} \times \vec{S}_1 \cdot \vec{v}_1 \vec{v}_1 \cdot \vec{v}_2 + \frac{7}{2} \hat{n} \times \vec{S}_1 \cdot \vec{v}_1 \vec{v}_2 \cdot \vec{v}_2 + 15 \hat{n} \times \vec{S}_1 \cdot \vec{v}_1 (\hat{n} \cdot \vec{v}_2)^2 \log\left(\frac{r}{R_\theta}\right) - \right. \\ \left. 6 \vec{S}_1 \times \vec{v}_1 \cdot \vec{v}_2 \hat{n} \cdot \vec{v}_2 \log\left(\frac{r}{R_\theta}\right) + \frac{93}{70} \hat{n} \times \vec{S}_1 \cdot \vec{v}_1 \vec{v}_1 \cdot \vec{v}_1 \log\left(\frac{r}{R_\theta}\right) + \frac{9}{10} \hat{n} \times \vec{S}_1 \cdot \vec{v}_1 \vec{v}_1 \cdot \vec{v}_2 \log\left(\frac{r}{R_\theta}\right) - \right. \\ \left. 3 \hat{n} \times \vec{S}_1 \cdot \vec{v}_1 \vec{v}_2 \cdot \vec{v}_2 \log\left(\frac{r}{R_\theta}\right) + \frac{1}{\epsilon_d} \left( \frac{31}{14} \hat{n} \times \vec{S}_1 \cdot \vec{v}_1 (\hat{n} \cdot \vec{v}_1)^2 - \frac{3}{10} \vec{S}_1 \times \vec{v}_1 \cdot \vec{v}_2 \hat{n} \cdot \vec{v}_1 + \frac{3}{2} \hat{n} \times \vec{S}_1 \cdot \vec{v}_1 \hat{n} \cdot \vec{v}_2 \hat{n} \cdot \vec{v}_1 - \right. \right. \\ \left. \left. 5 \hat{n} \times \vec{S}_1 \cdot \vec{v}_1 (\hat{n} \cdot \vec{v}_2)^2 + 2 \vec{S}_1 \times \vec{v}_1 \cdot \vec{v}_2 \hat{n} \cdot \vec{v}_2 - \frac{31}{70} \hat{n} \times \vec{S}_1 \cdot \vec{v}_1 \vec{v}_1 \cdot \vec{v}_1 - \frac{3}{10} \hat{n} \times \vec{S}_1 \cdot \vec{v}_1 \vec{v}_1 \cdot \vec{v}_2 + \hat{n} \times \vec{S}_1 \cdot \vec{v}_1 \vec{v}_2 \cdot \vec{v}_2 \right) \right) G^3 \Bigg\}$$

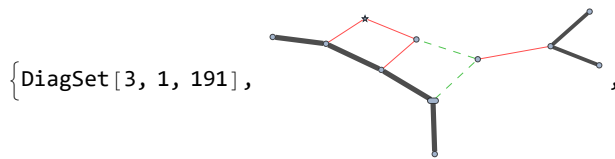

$$\frac{1}{r^3} G^3 m_1^2 m_2 \left( \frac{1}{\epsilon_d} \left( -\frac{1}{5} \hat{n} \cdot \vec{a}_1 \hat{n} \times \vec{S}_1 \cdot \vec{v}_1 - \frac{2}{5} \hat{n} \cdot \vec{v}_1 \hat{n} \times \vec{S}_1 \cdot \vec{a}_1 + \hat{n} \cdot \vec{v}_2 \hat{n} \times \vec{S}_1 \cdot \vec{a}_1 - \frac{1}{3} \vec{S}_1 \times \vec{a}_1 \cdot \vec{v}_2 - \frac{1}{15} \vec{S}_1 \times \vec{v}_1 \cdot \vec{a}_1 \right) + \right. \\ \left. \frac{3}{5} \log\left(\frac{r}{R_\theta}\right) \hat{n} \cdot \vec{a}_1 \hat{n} \times \vec{S}_1 \cdot \vec{v}_1 + \frac{6}{5} \log\left(\frac{r}{R_\theta}\right) \hat{n} \cdot \vec{v}_1 \hat{n} \times \vec{S}_1 \cdot \vec{a}_1 - 3 \log\left(\frac{r}{R_\theta}\right) \hat{n} \cdot \vec{v}_2 \hat{n} \times \vec{S}_1 \cdot \vec{a}_1 + \right. \\ \left. \frac{11}{50} \hat{n} \cdot \vec{a}_1 \hat{n} \times \vec{S}_1 \cdot \vec{v}_1 - \frac{54}{25} \hat{n} \cdot \vec{v}_1 \hat{n} \times \vec{S}_1 \cdot \vec{a}_1 + \frac{7}{2} \hat{n} \cdot \vec{v}_2 \hat{n} \times \vec{S}_1 \cdot \vec{a}_1 + \log\left(\frac{r}{R_\theta}\right) \vec{S}_1 \times \vec{a}_1 \cdot \vec{v}_2 + \right. \\ \left. \frac{1}{5} \log\left(\frac{r}{R_\theta}\right) \vec{S}_1 \times \vec{v}_1 \cdot \vec{a}_1 - \frac{5}{6} \vec{S}_1 \times \vec{a}_1 \cdot \vec{v}_2 - \frac{49}{150} \vec{S}_1 \times \vec{v}_1 \cdot \vec{a}_1 - \frac{1}{5} \hat{n} \cdot \vec{v}_1 \hat{n} \times \vec{S}_1 \cdot \vec{v}_1 \right) + \\ \frac{G^3 m_1^2 m_2 \left( \frac{\hat{n} \times \vec{S}_1 \cdot \vec{a}_1}{3 \epsilon_d} - \log\left(\frac{r}{R_\theta}\right) \hat{n} \times \vec{S}_1 \cdot \vec{a}_1 + \frac{5}{6} \hat{n} \times \vec{S}_1 \cdot \vec{a}_1 \right)}{r^2} + \frac{1}{r^4} G^3 m_1^2 m_2 \\ \left( \frac{\frac{2}{35} \vec{v}_1 \cdot \vec{v}_1 \hat{n} \times \vec{S}_1 \cdot \vec{v}_1 - \frac{2}{7} (\hat{n} \cdot \vec{v}_1)^2 \hat{n} \times \vec{S}_1 \cdot \vec{v}_1}{\epsilon_d} + \frac{6}{7} \log\left(\frac{r}{R_\theta}\right) (\hat{n} \cdot \vec{v}_1)^2 \hat{n} \times \vec{S}_1 \cdot \vec{v}_1 - \frac{6}{35} \log\left(\frac{r}{R_\theta}\right) \vec{v}_1 \cdot \vec{v}_1 \hat{n} \times \vec{S}_1 \cdot \vec{v}_1 - \right. \\ \left. \frac{22}{49} (\hat{n} \cdot \vec{v}_1)^2 \hat{n} \times \vec{S}_1 \cdot \vec{v}_1 + \frac{1}{5} \hat{n} \cdot \vec{v}_1 \vec{S}_1 \times \vec{v}_1 \cdot \vec{v}_2 - \hat{n} \cdot \vec{v}_2 \hat{n} \cdot \vec{v}_1 \hat{n} \times \vec{S}_1 \cdot \vec{v}_1 - \frac{247 \vec{v}_1 \cdot \vec{v}_1 \hat{n} \times \vec{S}_1 \cdot \vec{v}_1}{1225} + \frac{1}{5} \vec{v}_1 \cdot \vec{v}_2 \hat{n} \times \vec{S}_1 \cdot \vec{v}_1 \right) \Bigg\}$$

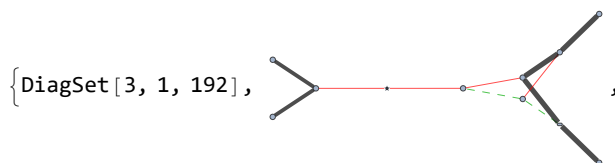

$$\frac{1}{r^3} G^3 m_1^2 m_2 \left( \frac{-\frac{1}{10} \hat{n} \cdot \vec{v}_2 \hat{n} \times \vec{S}_1 \cdot \vec{a}_1 + \frac{1}{30} \vec{S}_1 \times \vec{a}_1 \cdot \vec{v}_2 - \frac{1}{10} \hat{n} \cdot \vec{v}_2 \hat{n} \times \vec{S}_1 \cdot \vec{v}_1 + \frac{1}{30} \vec{S}_1 \times \vec{v}_1 \cdot \vec{v}_2}{\epsilon_d} + \right. \\ \left. \frac{3}{10} \log\left(\frac{r}{R_\theta}\right) \hat{n} \cdot \vec{v}_2 \hat{n} \times \vec{S}_1 \cdot \vec{a}_1 - \frac{7}{50} \hat{n} \cdot \vec{v}_2 \hat{n} \times \vec{S}_1 \cdot \vec{a}_1 - \frac{1}{10} \log\left(\frac{r}{R_\theta}\right) \vec{S}_1 \times \vec{a}_1 \cdot \vec{v}_2 + \frac{1}{75} \vec{S}_1 \times \vec{a}_1 \cdot \vec{v}_2 + \right. \\ \left. \frac{3}{10} \log\left(\frac{r}{R_\theta}\right) \hat{n} \cdot \vec{v}_2 \hat{n} \times \vec{S}_1 \cdot \vec{v}_1 - \frac{7}{50} \hat{n} \cdot \vec{v}_2 \hat{n} \times \vec{S}_1 \cdot \vec{v}_1 - \frac{1}{10} \log\left(\frac{r}{R_\theta}\right) \vec{S}_1 \times \vec{v}_1 \cdot \vec{v}_2 + \frac{1}{75} \vec{S}_1 \times \vec{v}_1 \cdot \vec{v}_2 \right) +$$

$$\frac{1}{r^4} G^3 m_1^2 m_2 \left( \frac{-\frac{1}{10} \hat{n} \cdot \vec{v}_1 \vec{S}_1 \times \vec{v}_1 \cdot \vec{v}_2 + \frac{1}{2} \hat{n} \cdot \vec{v}_2 \hat{n} \cdot \vec{v}_1 \hat{n} \times \vec{S}_1 \cdot \vec{v}_1 - \frac{1}{10} \vec{v}_1 \cdot \vec{v}_2 \hat{n} \times \vec{S}_1 \cdot \vec{v}_1}{\epsilon_d} + \right. \\ \left. \frac{3}{10} \log\left(\frac{r}{R_\theta}\right) \hat{n} \cdot \vec{v}_1 \vec{S}_1 \times \vec{v}_1 \cdot \vec{v}_2 - \frac{3}{2} \log\left(\frac{r}{R_\theta}\right) \hat{n} \cdot \vec{v}_2 \hat{n} \cdot \vec{v}_1 \hat{n} \times \vec{S}_1 \cdot \vec{v}_1 + \frac{3}{10} \log\left(\frac{r}{R_\theta}\right) \vec{v}_1 \cdot \vec{v}_2 \hat{n} \times \vec{S}_1 \cdot \vec{v}_1 - \right. \\ \left. \frac{7}{50} \hat{n} \cdot \vec{v}_1 \vec{S}_1 \times \vec{v}_1 \cdot \vec{v}_2 + \hat{n} \cdot \vec{v}_2 \hat{n} \cdot \vec{v}_1 \hat{n} \times \vec{S}_1 \cdot \vec{v}_1 - \frac{7}{50} \vec{v}_1 \cdot \vec{v}_2 \hat{n} \times \vec{S}_1 \cdot \vec{v}_1 \right) \Bigg\}$$

{DiagSet[3, 1, 193],

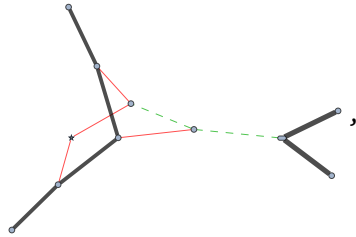

$$\frac{1}{r^3} G^3 m_2^3 \left( \frac{-\hat{n} \cdot \vec{a}_2 \hat{n} \times \vec{S}_1 \cdot \vec{v}_2 - \hat{n} \cdot \vec{v}_2 \hat{n} \times \vec{a}_2 \cdot \vec{S}_1 + \frac{2}{3} \vec{a}_2 \times \vec{S}_1 \cdot \vec{v}_2}{\epsilon_d} + 3 \log\left(\frac{r}{R_\theta}\right) \hat{n} \cdot \vec{a}_2 \hat{n} \times \vec{S}_1 \cdot \vec{v}_2 + 3 \log\left(\frac{r}{R_\theta}\right) \hat{n} \cdot \vec{v}_2 \hat{n} \times \vec{a}_2 \cdot \vec{S}_1 + \right. \\ \left. \frac{3}{2} \hat{n} \cdot \vec{a}_2 \hat{n} \times \vec{S}_1 \cdot \vec{v}_2 - 6 \hat{n} \cdot \vec{v}_1 \hat{n} \times \vec{a}_2 \cdot \vec{S}_1 + \frac{7}{2} \hat{n} \cdot \vec{v}_2 \hat{n} \times \vec{a}_2 \cdot \vec{S}_1 - 2 \log\left(\frac{r}{R_\theta}\right) \vec{a}_2 \times \vec{S}_1 \cdot \vec{v}_2 + 2 \vec{a}_2 \times \vec{S}_1 \cdot \vec{v}_1 - \frac{7}{3} \vec{a}_2 \times \vec{S}_1 \cdot \vec{v}_2 \right) + \\ \left. \frac{2 G^3 m_2^3 \hat{n} \times \vec{a}_2 \cdot \vec{S}_1}{r^2} + \frac{G^3 m_2^3 \left( 4 (\hat{n} \cdot \vec{v}_2)^2 \hat{n} \times \vec{S}_1 \cdot \vec{v}_2 + 2 \vec{v}_2 \cdot \vec{v}_2 \hat{n} \times \vec{S}_1 \cdot \vec{v}_2 \right)}{r^4} \right\}$$

{DiagSet[3, 1, 194],

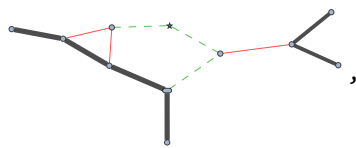

$$m_1^2 m_2 \left( \frac{1}{2} \log\left(\frac{r}{R_\theta}\right) \hat{n} \times \vec{S}_1 \cdot \vec{a}_1 - \frac{\hat{n} \times \vec{S}_1 \cdot \vec{a}_1}{6 \epsilon_d} - \frac{1}{3} \hat{n} \times \vec{S}_1 \cdot \vec{a}_1 \right) G^3 + \frac{1}{r^3}$$

$$m_1^2 m_2 \left( -\frac{1}{2} \log\left(\frac{r}{R_\theta}\right) \vec{S}_1 \times \vec{a}_1 \cdot \vec{v}_2 + \frac{1}{3} \vec{S}_1 \times \vec{a}_1 \cdot \vec{v}_2 + \frac{13}{25} \vec{S}_1 \times \vec{v}_1 \cdot \vec{a}_1 - \frac{13}{25} \hat{n} \times \vec{S}_1 \cdot \vec{v}_1 \hat{n} \cdot \vec{a}_1 + \frac{17}{25} \hat{n} \times \vec{S}_1 \cdot \vec{v}_1 \hat{n} \cdot \vec{v}_1 + \right. \\ \left. \frac{67}{50} \hat{n} \times \vec{S}_1 \cdot \vec{a}_1 \hat{n} \cdot \vec{v}_1 - \frac{3}{2} \hat{n} \times \vec{S}_1 \cdot \vec{a}_1 \hat{n} \cdot \vec{v}_2 - \frac{9}{10} \vec{S}_1 \times \vec{v}_1 \cdot \vec{a}_1 \log\left(\frac{r}{R_\theta}\right) + \frac{9}{10} \hat{n} \times \vec{S}_1 \cdot \vec{v}_1 \hat{n} \cdot \vec{a}_1 \log\left(\frac{r}{R_\theta}\right) - \right. \\ \left. \frac{3}{5} \hat{n} \times \vec{S}_1 \cdot \vec{v}_1 \hat{n} \cdot \vec{v}_1 \log\left(\frac{r}{R_\theta}\right) - \frac{9}{5} \hat{n} \times \vec{S}_1 \cdot \vec{a}_1 \hat{n} \cdot \vec{v}_1 \log\left(\frac{r}{R_\theta}\right) + \frac{3}{2} \hat{n} \times \vec{S}_1 \cdot \vec{a}_1 \hat{n} \cdot \vec{v}_2 \log\left(\frac{r}{R_\theta}\right) + \frac{1}{\epsilon_d} \right. \\ \left. \left( \frac{1}{6} \vec{S}_1 \times \vec{a}_1 \cdot \vec{v}_2 + \frac{3}{10} \vec{S}_1 \times \vec{v}_1 \cdot \vec{a}_1 - \frac{3}{10} \hat{n} \times \vec{S}_1 \cdot \vec{v}_1 \hat{n} \cdot \vec{a}_1 + \frac{1}{5} \hat{n} \times \vec{S}_1 \cdot \vec{v}_1 \hat{n} \cdot \vec{v}_1 + \frac{3}{5} \hat{n} \times \vec{S}_1 \cdot \vec{a}_1 \hat{n} \cdot \vec{v}_1 - \frac{1}{2} \hat{n} \times \vec{S}_1 \cdot \vec{a}_1 \hat{n} \cdot \vec{v}_2 \right) \right) \\ G^3 + \frac{1}{r^4} m_1^2 m_2 \left( -\frac{82}{49} \hat{n} \times \vec{S}_1 \cdot \vec{v}_1 (\hat{n} \cdot \vec{v}_1)^2 + \frac{9}{7} \hat{n} \times \vec{S}_1 \cdot \vec{v}_1 \log\left(\frac{r}{R_\theta}\right) (\hat{n} \cdot \vec{v}_1)^2 - \frac{17}{25} \vec{S}_1 \times \vec{v}_1 \cdot \vec{v}_2 \hat{n} \cdot \vec{v}_1 + \right. \\ \left. 4 \hat{n} \times \vec{S}_1 \cdot \vec{v}_1 \hat{n} \cdot \vec{v}_2 \hat{n} \cdot \vec{v}_1 + \frac{3}{5} \vec{S}_1 \times \vec{v}_1 \cdot \vec{v}_2 \log\left(\frac{r}{R_\theta}\right) \hat{n} \cdot \vec{v}_1 - 3 \hat{n} \times \vec{S}_1 \cdot \vec{v}_1 \hat{n} \cdot \vec{v}_2 \log\left(\frac{r}{R_\theta}\right) \hat{n} \cdot \vec{v}_1 + \frac{242 \hat{n} \times \vec{S}_1 \cdot \vec{v}_1 \vec{v}_1 \cdot \vec{v}_1}{1225} - \right. \\ \left. \frac{17}{25} \hat{n} \times \vec{S}_1 \cdot \vec{v}_1 \vec{v}_1 \cdot \vec{v}_2 - \frac{9}{35} \hat{n} \times \vec{S}_1 \cdot \vec{v}_1 \vec{v}_1 \cdot \vec{v}_1 \log\left(\frac{r}{R_\theta}\right) + \frac{3}{5} \hat{n} \times \vec{S}_1 \cdot \vec{v}_1 \vec{v}_1 \cdot \vec{v}_2 \log\left(\frac{r}{R_\theta}\right) + \frac{1}{\epsilon_d} \left( -\frac{3}{7} \hat{n} \times \vec{S}_1 \cdot \vec{v}_1 (\hat{n} \cdot \vec{v}_1)^2 - \right. \right. \\ \left. \left. \frac{1}{5} \vec{S}_1 \times \vec{v}_1 \cdot \vec{v}_2 \hat{n} \cdot \vec{v}_1 + \hat{n} \times \vec{S}_1 \cdot \vec{v}_1 \hat{n} \cdot \vec{v}_2 \hat{n} \cdot \vec{v}_1 + \frac{3}{35} \hat{n} \times \vec{S}_1 \cdot \vec{v}_1 \vec{v}_1 \cdot \vec{v}_1 - \frac{1}{5} \hat{n} \times \vec{S}_1 \cdot \vec{v}_1 \vec{v}_1 \cdot \vec{v}_2 \right) \right) G^3 \Bigg\}$$

{DiagSet[3, 1, 195],

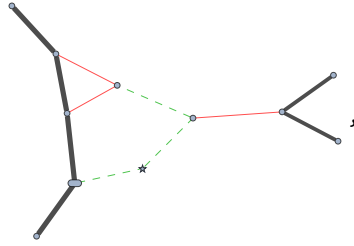

$$\frac{m_1^2 m_2 \left( -\frac{1}{2} \log\left(\frac{r}{R_0}\right) \hat{n} \times \vec{S}_1 \cdot \vec{a}_1 + \frac{\hat{n} \times \vec{S}_1 \cdot \vec{a}_1}{6 \in_d} - \frac{1}{6} \hat{n} \times \vec{S}_1 \cdot \vec{a}_1 \right) G^3}{r^2} + \frac{1}{r^3} m_1^2 m_2 \left( \frac{1}{2} \log\left(\frac{r}{R_0}\right) \vec{S}_1 \times \vec{v}_1 \cdot \vec{v}_2 + \frac{1}{6} \vec{S}_1 \times \vec{v}_1 \cdot \vec{v}_2 + \right. \\ \left. \frac{9}{50} \vec{S}_1 \times \vec{v}_1 \cdot \vec{a}_1 - \frac{7}{50} \hat{n} \times \vec{S}_1 \cdot \vec{v}_1 \hat{n} \cdot \vec{a}_1 + \frac{1}{25} \hat{n} \times \vec{S}_1 \cdot \vec{v}_1 \hat{n} \cdot \vec{v}_1 + \frac{1}{10} \hat{n} \times \vec{S}_1 \cdot \vec{a}_1 \hat{n} \cdot \vec{v}_1 - \frac{1}{10} \vec{S}_1 \times \vec{v}_1 \cdot \vec{a}_1 \log\left(\frac{r}{R_0}\right) + \right. \\ \left. \frac{3}{10} \hat{n} \times \vec{S}_1 \cdot \vec{v}_1 \hat{n} \cdot \vec{a}_1 \log\left(\frac{r}{R_0}\right) + \frac{6}{5} \hat{n} \times \vec{S}_1 \cdot \vec{v}_1 \hat{n} \cdot \vec{v}_1 \log\left(\frac{r}{R_0}\right) - \frac{3}{2} \hat{n} \times \vec{S}_1 \cdot \vec{v}_1 \hat{n} \cdot \vec{v}_2 \log\left(\frac{r}{R_0}\right) + \frac{1}{\in_d} \right. \\ \left. \left( -\frac{1}{6} \vec{S}_1 \times \vec{v}_1 \cdot \vec{v}_2 + \frac{1}{30} \vec{S}_1 \times \vec{v}_1 \cdot \vec{a}_1 - \frac{1}{10} \hat{n} \times \vec{S}_1 \cdot \vec{v}_1 \hat{n} \cdot \vec{a}_1 - \frac{2}{5} \hat{n} \times \vec{S}_1 \cdot \vec{v}_1 \hat{n} \cdot \vec{v}_1 + \frac{1}{2} \hat{n} \times \vec{S}_1 \cdot \vec{v}_1 \hat{n} \cdot \vec{v}_2 \right) \right) G^3 + \frac{1}{r^4} \\ m_1^2 m_2 \left( \frac{15}{49} \hat{n} \times \vec{S}_1 \cdot \vec{v}_1 (\hat{n} \cdot \vec{v}_1)^2 - \frac{6}{7} \hat{n} \times \vec{S}_1 \cdot \vec{v}_1 \log\left(\frac{r}{R_0}\right) (\hat{n} \cdot \vec{v}_1)^2 + \frac{1}{25} \vec{S}_1 \times \vec{v}_1 \cdot \vec{v}_2 \hat{n} \cdot \vec{v}_1 - \frac{1}{2} \hat{n} \times \vec{S}_1 \cdot \vec{v}_1 \hat{n} \cdot \vec{v}_2 \hat{n} \cdot \vec{v}_1 - \right. \\ \left. \frac{3}{10} \vec{S}_1 \times \vec{v}_1 \cdot \vec{v}_2 \log\left(\frac{r}{R_0}\right) \hat{n} \cdot \vec{v}_1 + \frac{3}{2} \hat{n} \times \vec{S}_1 \cdot \vec{v}_1 \hat{n} \cdot \vec{v}_2 \log\left(\frac{r}{R_0}\right) \hat{n} \cdot \vec{v}_1 + \frac{37 \hat{n} \times \vec{S}_1 \cdot \vec{v}_1 \vec{v}_1 \cdot \vec{v}_1}{1225} + \frac{1}{25} \hat{n} \times \vec{S}_1 \cdot \vec{v}_1 \vec{v}_1 \cdot \vec{v}_2 + \right. \\ \left. \frac{6}{35} \hat{n} \times \vec{S}_1 \cdot \vec{v}_1 \vec{v}_1 \cdot \vec{v}_1 \log\left(\frac{r}{R_0}\right) - \frac{3}{10} \hat{n} \times \vec{S}_1 \cdot \vec{v}_1 \vec{v}_1 \cdot \vec{v}_2 \log\left(\frac{r}{R_0}\right) + \frac{1}{\in_d} \left( \frac{2}{7} \hat{n} \times \vec{S}_1 \cdot \vec{v}_1 (\hat{n} \cdot \vec{v}_1)^2 + \right. \right. \\ \left. \left. \frac{1}{10} \vec{S}_1 \times \vec{v}_1 \cdot \vec{v}_2 \hat{n} \cdot \vec{v}_1 - \frac{1}{2} \hat{n} \times \vec{S}_1 \cdot \vec{v}_1 \hat{n} \cdot \vec{v}_2 \hat{n} \cdot \vec{v}_1 - \frac{2}{35} \hat{n} \times \vec{S}_1 \cdot \vec{v}_1 \vec{v}_1 \cdot \vec{v}_1 + \frac{1}{10} \hat{n} \times \vec{S}_1 \cdot \vec{v}_1 \vec{v}_1 \cdot \vec{v}_2 \right) \right) G^3 \Big\}$$

{DiagSet[3, 1, 196],

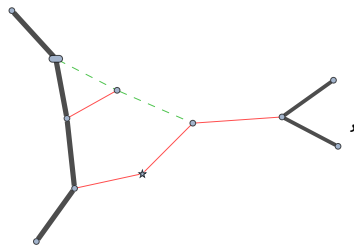

$$\frac{m_1^2 m_2 \left( -\frac{1}{2} \log\left(\frac{r}{R_0}\right) \hat{n} \times \vec{S}_1 \cdot \vec{a}_1 + \frac{\hat{n} \times \vec{S}_1 \cdot \vec{a}_1}{6 \in_d} + \frac{1}{6} \hat{n} \times \vec{S}_1 \cdot \vec{a}_1 \right) G^3}{r^2} + \frac{1}{r^3} m_1^2 m_2 \left( -\frac{1}{2} \log\left(\frac{r}{R_0}\right) \vec{S}_1 \times \vec{v}_1 \cdot \vec{v}_2 + \frac{1}{6} \vec{S}_1 \times \vec{v}_1 \cdot \vec{v}_2 - \right. \\ \left. \frac{1}{6} \vec{S}_1 \times \vec{a}_1 \cdot \vec{v}_2 - \frac{1}{6} \vec{S}_1 \times \vec{v}_1 \cdot \vec{a}_1 + \frac{1}{6} \vec{S}_1 \times \vec{v}_1 \cdot \vec{a}_2 + \frac{6}{25} \hat{n} \times \vec{S}_1 \cdot \vec{v}_1 \hat{n} \cdot \vec{a}_1 - \hat{n} \times \vec{S}_1 \cdot \vec{v}_1 \hat{n} \cdot \vec{a}_2 - \frac{12}{25} \hat{n} \times \vec{S}_1 \cdot \vec{v}_1 \hat{n} \cdot \vec{v}_1 - \right. \\ \left. \frac{19}{25} \hat{n} \times \vec{S}_1 \cdot \vec{a}_1 \hat{n} \cdot \vec{v}_1 - \hat{n} \times \vec{S}_1 \cdot \vec{v}_1 \hat{n} \cdot \vec{v}_2 + \hat{n} \times \vec{S}_1 \cdot \vec{a}_1 \hat{n} \cdot \vec{v}_2 + \frac{1}{2} \vec{S}_1 \times \vec{a}_1 \cdot \vec{v}_2 \log\left(\frac{r}{R_0}\right) + \frac{1}{2} \vec{S}_1 \times \vec{v}_1 \cdot \vec{a}_1 \log\left(\frac{r}{R_0}\right) - \right. \\ \left. \frac{1}{2} \vec{S}_1 \times \vec{v}_1 \cdot \vec{a}_2 \log\left(\frac{r}{R_0}\right) - \frac{3}{10} \hat{n} \times \vec{S}_1 \cdot \vec{v}_1 \hat{n} \cdot \vec{a}_1 \log\left(\frac{r}{R_0}\right) + \frac{3}{2} \hat{n} \times \vec{S}_1 \cdot \vec{v}_1 \hat{n} \cdot \vec{a}_2 \log\left(\frac{r}{R_0}\right) + \frac{3}{5} \hat{n} \times \vec{S}_1 \cdot \vec{v}_1 \hat{n} \cdot \vec{v}_1 \log\left(\frac{r}{R_0}\right) + \right. \\ \left. \frac{6}{5} \hat{n} \times \vec{S}_1 \cdot \vec{a}_1 \hat{n} \cdot \vec{v}_1 \log\left(\frac{r}{R_0}\right) + \frac{3}{2} \hat{n} \times \vec{S}_1 \cdot \vec{v}_1 \hat{n} \cdot \vec{v}_2 \log\left(\frac{r}{R_0}\right) - \frac{3}{2} \hat{n} \times \vec{S}_1 \cdot \vec{a}_1 \hat{n} \cdot \vec{v}_2 \log\left(\frac{r}{R_0}\right) + \frac{1}{\in_d} \right. \\ \left. \left( \frac{1}{6} \vec{S}_1 \times \vec{v}_1 \cdot \vec{v}_2 - \frac{1}{6} \vec{S}_1 \times \vec{a}_1 \cdot \vec{v}_2 - \frac{1}{6} \vec{S}_1 \times \vec{v}_1 \cdot \vec{a}_1 + \frac{1}{6} \vec{S}_1 \times \vec{v}_1 \cdot \vec{a}_2 + \frac{1}{10} \hat{n} \times \vec{S}_1 \cdot \vec{v}_1 \hat{n} \cdot \vec{a}_1 - \frac{1}{2} \hat{n} \times \vec{S}_1 \cdot \vec{v}_1 \hat{n} \cdot \vec{a}_2 - \right. \right. \\ \left. \left. \frac{1}{5} \hat{n} \times \vec{S}_1 \cdot \vec{v}_1 \hat{n} \cdot \vec{v}_1 - \frac{2}{5} \hat{n} \times \vec{S}_1 \cdot \vec{a}_1 \hat{n} \cdot \vec{v}_1 - \frac{1}{2} \hat{n} \times \vec{S}_1 \cdot \vec{v}_1 \hat{n} \cdot \vec{v}_2 + \frac{1}{2} \hat{n} \times \vec{S}_1 \cdot \vec{a}_1 \hat{n} \cdot \vec{v}_2 \right) \right) G^3 + \frac{1}{r^4}$$

$$m_1^2 m_2 \left( \frac{111}{98} \hat{n} \times \vec{S}_1 \cdot \vec{v}_1 (\hat{n} \cdot \vec{v}_1)^2 - \frac{15}{14} \hat{n} \times \vec{S}_1 \cdot \vec{v}_1 \log\left(\frac{r}{R_0}\right) (\hat{n} \cdot \vec{v}_1)^2 - \frac{1}{25} \vec{S}_1 \times \vec{v}_1 \cdot \vec{v}_2 \hat{n} \cdot \vec{v}_1 + \frac{1}{2} \hat{n} \times \vec{S}_1 \cdot \vec{v}_1 \hat{n} \cdot \vec{v}_2 \hat{n} \cdot \vec{v}_1 + \right. \\ \left. \frac{3}{10} \vec{S}_1 \times \vec{v}_1 \cdot \vec{v}_2 \log\left(\frac{r}{R_0}\right) \hat{n} \cdot \vec{v}_1 - \frac{3}{2} \hat{n} \times \vec{S}_1 \cdot \vec{v}_1 \hat{n} \cdot \vec{v}_2 \log\left(\frac{r}{R_0}\right) \hat{n} \cdot \vec{v}_1 - \frac{13}{2} \hat{n} \times \vec{S}_1 \cdot \vec{v}_1 (\hat{n} \cdot \vec{v}_2)^2 + 2 \vec{S}_1 \times \vec{v}_1 \cdot \vec{v}_2 \hat{n} \cdot \vec{v}_2 - \right. \\ \left. \frac{3}{245} \hat{n} \times \vec{S}_1 \cdot \vec{v}_1 \vec{v}_1 \cdot \vec{v}_1 - \frac{1}{25} \hat{n} \times \vec{S}_1 \cdot \vec{v}_1 \vec{v}_1 \cdot \vec{v}_2 + \hat{n} \times \vec{S}_1 \cdot \vec{v}_1 \vec{v}_2 \cdot \vec{v}_2 + \frac{15}{2} \hat{n} \times \vec{S}_1 \cdot \vec{v}_1 (\hat{n} \cdot \vec{v}_2)^2 \log\left(\frac{r}{R_0}\right) - \right. \\ \left. 3 \vec{S}_1 \times \vec{v}_1 \cdot \vec{v}_2 \hat{n} \cdot \vec{v}_2 \log\left(\frac{r}{R_0}\right) + \frac{3}{14} \hat{n} \times \vec{S}_1 \cdot \vec{v}_1 \vec{v}_1 \cdot \vec{v}_1 \log\left(\frac{r}{R_0}\right) + \frac{3}{10} \hat{n} \times \vec{S}_1 \cdot \vec{v}_1 \vec{v}_1 \cdot \vec{v}_2 \log\left(\frac{r}{R_0}\right) - \right. \\ \left. \frac{3}{2} \hat{n} \times \vec{S}_1 \cdot \vec{v}_1 \vec{v}_2 \cdot \vec{v}_2 \log\left(\frac{r}{R_0}\right) + \frac{1}{\epsilon_d} \left( \frac{5}{14} \hat{n} \times \vec{S}_1 \cdot \vec{v}_1 (\hat{n} \cdot \vec{v}_1)^2 - \frac{1}{10} \vec{S}_1 \times \vec{v}_1 \cdot \vec{v}_2 \hat{n} \cdot \vec{v}_1 + \frac{1}{2} \hat{n} \times \vec{S}_1 \cdot \vec{v}_1 \hat{n} \cdot \vec{v}_2 \hat{n} \cdot \vec{v}_1 - \right. \right. \\ \left. \left. \frac{5}{2} \hat{n} \times \vec{S}_1 \cdot \vec{v}_1 (\hat{n} \cdot \vec{v}_2)^2 + \vec{S}_1 \times \vec{v}_1 \cdot \vec{v}_2 \hat{n} \cdot \vec{v}_2 - \frac{1}{14} \hat{n} \times \vec{S}_1 \cdot \vec{v}_1 \vec{v}_1 \cdot \vec{v}_1 - \frac{1}{10} \hat{n} \times \vec{S}_1 \cdot \vec{v}_1 \vec{v}_1 \cdot \vec{v}_2 + \frac{1}{2} \hat{n} \times \vec{S}_1 \cdot \vec{v}_1 \vec{v}_2 \cdot \vec{v}_2 \right) \right) G^3 \Big\}$$

{DiagSet[3, 1, 197],

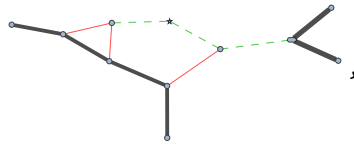

$$\frac{1}{r^3} G^3 m_2^3 \left( \frac{-\frac{1}{2} \hat{n} \cdot \vec{a}_2 \hat{n} \times \vec{S}_1 \cdot \vec{v}_2 - \frac{1}{2} \hat{n} \cdot \vec{v}_2 \hat{n} \times \vec{a}_2 \cdot \vec{S}_1 + \frac{1}{3} \vec{a}_2 \times \vec{S}_1 \cdot \vec{v}_2}{\epsilon_d} + \frac{3}{2} \log\left(\frac{r}{R_0}\right) \hat{n} \cdot \vec{a}_2 \hat{n} \times \vec{S}_1 \cdot \vec{v}_2 + \right. \\ \left. \frac{3}{2} \log\left(\frac{r}{R_0}\right) \hat{n} \cdot \vec{v}_2 \hat{n} \times \vec{a}_2 \cdot \vec{S}_1 - \hat{n} \cdot \vec{a}_2 \hat{n} \times \vec{S}_1 \cdot \vec{v}_2 + 3 \hat{n} \cdot \vec{v}_1 \hat{n} \times \vec{a}_2 \cdot \vec{S}_1 - 2 \hat{n} \cdot \vec{v}_2 \hat{n} \times \vec{a}_2 \cdot \vec{S}_1 - \right. \\ \left. \log\left(\frac{r}{R_0}\right) \vec{a}_2 \times \vec{S}_1 \cdot \vec{v}_2 - \left( \vec{a}_2 \times \vec{S}_1 \cdot \vec{v}_1 \right) + \frac{2}{3} \vec{a}_2 \times \vec{S}_1 \cdot \vec{v}_2 + 2 \hat{n} \cdot \vec{v}_2 \hat{n} \times \vec{S}_1 \cdot \vec{v}_2 \right) - \frac{G^3 m_2^3 \hat{n} \times \vec{a}_2 \cdot \vec{S}_1}{r^2} + \\ \left. \frac{1}{r^4} G^3 m_2^3 \left( 2 (\hat{n} \cdot \vec{v}_2)^2 \hat{n} \times \vec{S}_1 \cdot \vec{v}_2 - 2 \hat{n} \cdot \vec{v}_2 \vec{S}_1 \times \vec{v}_1 \cdot \vec{v}_2 - 10 \hat{n} \cdot \vec{v}_1 \hat{n} \cdot \vec{v}_2 \hat{n} \times \vec{S}_1 \cdot \vec{v}_2 + 2 \vec{v}_1 \cdot \vec{v}_2 \hat{n} \times \vec{S}_1 \cdot \vec{v}_2 \right) \right\}$$

{DiagSet[3, 1, 198],

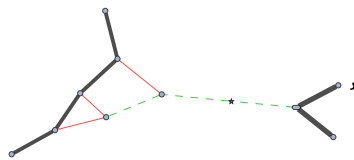

$$\frac{1}{r^3} G^3 m_2^3 \left( \frac{-\hat{n} \cdot \vec{v}_1 \hat{n} \times \vec{a}_2 \cdot \vec{S}_1 + \frac{1}{3} \vec{a}_2 \times \vec{S}_1 \cdot \vec{v}_1 - \hat{n} \cdot \vec{v}_2 \hat{n} \times \vec{S}_1 \cdot \vec{v}_2}{\epsilon_d} + 3 \log\left(\frac{r}{R_0}\right) \hat{n} \cdot \vec{v}_1 \hat{n} \times \vec{a}_2 \cdot \vec{S}_1 + \hat{n} \cdot \vec{v}_1 \left( -(\hat{n} \times \vec{a}_2 \cdot \vec{S}_1) \right) - \right. \\ \left. \log\left(\frac{r}{R_0}\right) \vec{a}_2 \times \vec{S}_1 \cdot \vec{v}_1 + 3 \log\left(\frac{r}{R_0}\right) \hat{n} \cdot \vec{v}_2 \hat{n} \times \vec{S}_1 \cdot \vec{v}_2 - \hat{n} \cdot \vec{v}_2 \hat{n} \times \vec{S}_1 \cdot \vec{v}_2 \right) + \frac{G^3 m_2^3 \left( \frac{\hat{n} \times \vec{a}_2 \cdot \vec{S}_1}{3 \epsilon_d} - \log\left(\frac{r}{R_0}\right) \hat{n} \times \vec{a}_2 \cdot \vec{S}_1 \right)}{r^2} + \frac{1}{r^4} \\ G^3 m_2^3 \left( \frac{\hat{n} \cdot \vec{v}_2 \vec{S}_1 \times \vec{v}_1 \cdot \vec{v}_2 + 5 \hat{n} \cdot \vec{v}_1 \hat{n} \cdot \vec{v}_2 \hat{n} \times \vec{S}_1 \cdot \vec{v}_2 - \vec{v}_1 \cdot \vec{v}_2 \hat{n} \times \vec{S}_1 \cdot \vec{v}_2}{\epsilon_d} - 3 \log\left(\frac{r}{R_0}\right) \hat{n} \cdot \vec{v}_2 \vec{S}_1 \times \vec{v}_1 \cdot \vec{v}_2 - 15 \log\left(\frac{r}{R_0}\right) \hat{n} \cdot \vec{v}_1 \right. \\ \left. \hat{n} \cdot \vec{v}_2 \hat{n} \times \vec{S}_1 \cdot \vec{v}_2 + 3 \log\left(\frac{r}{R_0}\right) \vec{v}_1 \cdot \vec{v}_2 \hat{n} \times \vec{S}_1 \cdot \vec{v}_2 + \hat{n} \cdot \vec{v}_2 \vec{S}_1 \times \vec{v}_1 \cdot \vec{v}_2 + 8 \hat{n} \cdot \vec{v}_1 \hat{n} \cdot \vec{v}_2 \hat{n} \times \vec{S}_1 \cdot \vec{v}_2 - \vec{v}_1 \cdot \vec{v}_2 \hat{n} \times \vec{S}_1 \cdot \vec{v}_2 \right) \Big\}$$

{DiagSet[3, 1, 199], 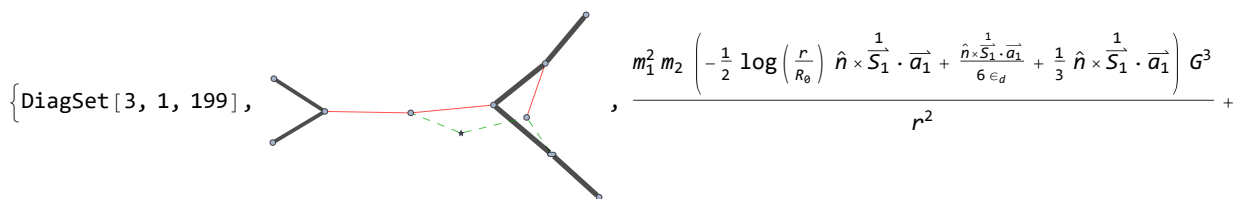 , 
$$\frac{m_1^2 m_2 \left( -\frac{1}{2} \log\left(\frac{r}{R_\theta}\right) \hat{n} \times \vec{S}_1 \cdot \vec{a}_1 + \frac{\hat{n} \times \vec{S}_1 \cdot \vec{a}_1}{6 \epsilon_d} + \frac{1}{3} \hat{n} \times \vec{S}_1 \cdot \vec{a}_1 \right) G^3}{r^2} +$$

$$\begin{aligned} & \frac{1}{r^3} m_1^2 m_2 \left( \frac{1}{2} \log\left(\frac{r}{R_\theta}\right) \vec{S}_1 \times \vec{v}_1 \cdot \vec{a}_1 - \frac{1}{3} \vec{S}_1 \times \vec{v}_1 \cdot \vec{a}_1 - \frac{1}{3} \vec{S}_1 \times \vec{v}_1 \cdot \vec{a}_2 + \frac{41}{50} \hat{n} \times \vec{S}_1 \cdot \vec{v}_1 \hat{n} \cdot \vec{a}_1 + \frac{3}{2} \hat{n} \times \vec{S}_1 \cdot \vec{v}_1 \hat{n} \cdot \vec{a}_2 - \right. \\ & \frac{41}{25} \hat{n} \times \vec{S}_1 \cdot \vec{v}_1 \hat{n} \cdot \vec{v}_1 - \frac{17}{25} \hat{n} \times \vec{S}_1 \cdot \vec{a}_1 \hat{n} \cdot \vec{v}_1 + \frac{1}{2} \vec{S}_1 \times \vec{v}_1 \cdot \vec{a}_2 \log\left(\frac{r}{R_\theta}\right) - \frac{9}{10} \hat{n} \times \vec{S}_1 \cdot \vec{v}_1 \hat{n} \cdot \vec{a}_1 \log\left(\frac{r}{R_\theta}\right) - \\ & \frac{3}{2} \hat{n} \times \vec{S}_1 \cdot \vec{v}_1 \hat{n} \cdot \vec{a}_2 \log\left(\frac{r}{R_\theta}\right) + \frac{9}{5} \hat{n} \times \vec{S}_1 \cdot \vec{v}_1 \hat{n} \cdot \vec{v}_1 \log\left(\frac{r}{R_\theta}\right) + \frac{3}{5} \hat{n} \times \vec{S}_1 \cdot \vec{a}_1 \hat{n} \cdot \vec{v}_1 \log\left(\frac{r}{R_\theta}\right) + \frac{1}{\epsilon_d} \\ & \left. \left( -\frac{1}{6} \vec{S}_1 \times \vec{v}_1 \cdot \vec{a}_1 - \frac{1}{6} \vec{S}_1 \times \vec{v}_1 \cdot \vec{a}_2 + \frac{3}{10} \hat{n} \times \vec{S}_1 \cdot \vec{v}_1 \hat{n} \cdot \vec{a}_1 + \frac{1}{2} \hat{n} \times \vec{S}_1 \cdot \vec{v}_1 \hat{n} \cdot \vec{a}_2 - \frac{3}{5} \hat{n} \times \vec{S}_1 \cdot \vec{v}_1 \hat{n} \cdot \vec{v}_1 - \frac{1}{5} \hat{n} \times \vec{S}_1 \cdot \vec{a}_1 \hat{n} \cdot \vec{v}_1 \right) \right) \\ & G^3 + \frac{1}{r^4} m_1^2 m_2 \left( \frac{1}{49} \hat{n} \times \vec{S}_1 \cdot \vec{v}_1 (\hat{n} \cdot \vec{v}_1)^2 + \frac{9}{14} \hat{n} \times \vec{S}_1 \cdot \vec{v}_1 \log\left(\frac{r}{R_\theta}\right) (\hat{n} \cdot \vec{v}_1)^2 + 9 \hat{n} \times \vec{S}_1 \cdot \vec{v}_1 (\hat{n} \cdot \vec{v}_2)^2 - 3 \vec{S}_1 \times \vec{v}_1 \cdot \vec{v}_2 \hat{n} \cdot \vec{v}_2 + \right. \\ & \frac{557 \hat{n} \times \vec{S}_1 \cdot \vec{v}_1 \vec{v}_1 \cdot \vec{v}_1}{2450} - \frac{3}{2} \hat{n} \times \vec{S}_1 \cdot \vec{v}_1 \vec{v}_2 \cdot \vec{v}_2 - \frac{15}{2} \hat{n} \times \vec{S}_1 \cdot \vec{v}_1 (\hat{n} \cdot \vec{v}_2)^2 \log\left(\frac{r}{R_\theta}\right) + 3 \vec{S}_1 \times \vec{v}_1 \cdot \vec{v}_2 \hat{n} \cdot \vec{v}_2 \log\left(\frac{r}{R_\theta}\right) - \\ & \frac{9}{70} \hat{n} \times \vec{S}_1 \cdot \vec{v}_1 \vec{v}_1 \cdot \vec{v}_1 \log\left(\frac{r}{R_\theta}\right) + \frac{3}{2} \hat{n} \times \vec{S}_1 \cdot \vec{v}_1 \vec{v}_2 \cdot \vec{v}_2 \log\left(\frac{r}{R_\theta}\right) + \frac{1}{\epsilon_d} \left( -\frac{3}{14} \hat{n} \times \vec{S}_1 \cdot \vec{v}_1 (\hat{n} \cdot \vec{v}_1)^2 + \right. \\ & \left. \left. \frac{5}{2} \hat{n} \times \vec{S}_1 \cdot \vec{v}_1 (\hat{n} \cdot \vec{v}_2)^2 - \vec{S}_1 \times \vec{v}_1 \cdot \vec{v}_2 \hat{n} \cdot \vec{v}_2 + \frac{3}{70} \hat{n} \times \vec{S}_1 \cdot \vec{v}_1 \vec{v}_1 \cdot \vec{v}_1 - \frac{1}{2} \hat{n} \times \vec{S}_1 \cdot \vec{v}_1 \vec{v}_2 \cdot \vec{v}_2 \right) \right) G^3 \} \end{aligned}$$

{DiagSet[3, 1, 200], 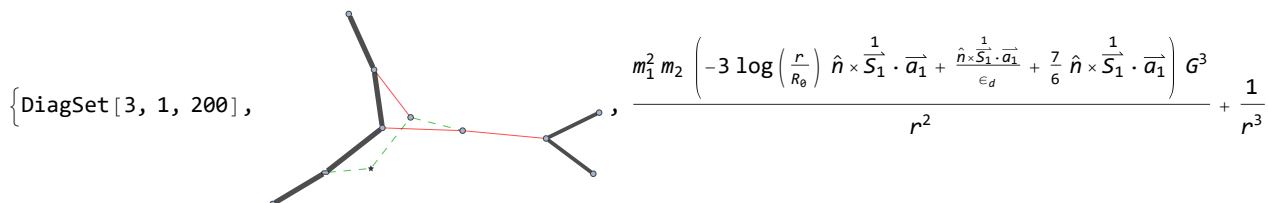 , 
$$\frac{m_1^2 m_2 \left( -3 \log\left(\frac{r}{R_\theta}\right) \hat{n} \times \vec{S}_1 \cdot \vec{a}_1 + \frac{\hat{n} \times \vec{S}_1 \cdot \vec{a}_1}{\epsilon_d} + \frac{7}{6} \hat{n} \times \vec{S}_1 \cdot \vec{a}_1 \right) G^3}{r^2} + \frac{1}{r^3}$$

$$\begin{aligned} & m_1^2 m_2 \left( \log\left(\frac{r}{R_\theta}\right) \frac{1}{\vec{S}_1 \times \vec{v}_1 \cdot \vec{v}_2} - \frac{1}{6} \frac{1}{\vec{S}_1 \times \vec{v}_1 \cdot \vec{v}_2} - \frac{33}{50} \vec{S}_1 \times \vec{v}_1 \cdot \vec{a}_1 - \vec{S}_1 \times \vec{v}_1 \cdot \vec{a}_2 + \frac{117}{50} \hat{n} \times \vec{S}_1 \cdot \vec{v}_1 \hat{n} \cdot \vec{a}_1 + 5 \hat{n} \times \vec{S}_1 \cdot \vec{v}_1 \hat{n} \cdot \vec{a}_2 - \right. \\ & \frac{73}{10} \hat{n} \times \vec{S}_1 \cdot \vec{v}_1 \hat{n} \cdot \vec{v}_1 - \frac{77}{50} \hat{n} \times \vec{S}_1 \cdot \vec{a}_1 \hat{n} \cdot \vec{v}_1 + \frac{3}{2} \hat{n} \times \vec{S}_1 \cdot \vec{v}_1 \hat{n} \cdot \vec{v}_2 + \frac{17}{10} \vec{S}_1 \times \vec{v}_1 \cdot \vec{a}_1 \log\left(\frac{r}{R_\theta}\right) + 2 \vec{S}_1 \times \vec{v}_1 \cdot \vec{a}_2 \log\left(\frac{r}{R_\theta}\right) - \\ & \frac{33}{10} \hat{n} \times \vec{S}_1 \cdot \vec{v}_1 \hat{n} \cdot \vec{a}_1 \log\left(\frac{r}{R_\theta}\right) - 6 \hat{n} \times \vec{S}_1 \cdot \vec{v}_1 \hat{n} \cdot \vec{a}_2 \log\left(\frac{r}{R_\theta}\right) + \frac{21}{2} \hat{n} \times \vec{S}_1 \cdot \vec{v}_1 \hat{n} \cdot \vec{v}_1 \log\left(\frac{r}{R_\theta}\right) + \\ & \frac{9}{5} \hat{n} \times \vec{S}_1 \cdot \vec{a}_1 \hat{n} \cdot \vec{v}_1 \log\left(\frac{r}{R_\theta}\right) - 3 \hat{n} \times \vec{S}_1 \cdot \vec{v}_1 \hat{n} \cdot \vec{v}_2 \log\left(\frac{r}{R_\theta}\right) + \frac{1}{\epsilon_d} \left( -\frac{1}{3} \frac{1}{\vec{S}_1 \times \vec{v}_1 \cdot \vec{v}_2} - \frac{17}{30} \vec{S}_1 \times \vec{v}_1 \cdot \vec{a}_1 - \frac{2}{3} \vec{S}_1 \times \vec{v}_1 \cdot \vec{a}_2 + \right. \\ & \left. \frac{11}{10} \hat{n} \times \vec{S}_1 \cdot \vec{v}_1 \hat{n} \cdot \vec{a}_1 + 2 \hat{n} \times \vec{S}_1 \cdot \vec{v}_1 \hat{n} \cdot \vec{a}_2 - \frac{7}{2} \hat{n} \times \vec{S}_1 \cdot \vec{v}_1 \hat{n} \cdot \vec{v}_1 - \frac{3}{5} \hat{n} \times \vec{S}_1 \cdot \vec{a}_1 \hat{n} \cdot \vec{v}_1 + \hat{n} \times \vec{S}_1 \cdot \vec{v}_1 \hat{n} \cdot \vec{v}_2 \right) \left. \right) G^3 + \\ & \frac{1}{r^4} m_1^2 m_2 \left( -\frac{16}{7} \hat{n} \times \vec{S}_1 \cdot \vec{v}_1 (\hat{n} \cdot \vec{v}_1)^2 + \frac{9}{2} \hat{n} \times \vec{S}_1 \cdot \vec{v}_1 \log\left(\frac{r}{R_\theta}\right) (\hat{n} \cdot \vec{v}_1)^2 + \frac{23}{25} \vec{S}_1 \times \vec{v}_1 \cdot \vec{v}_2 \hat{n} \cdot \vec{v}_1 - \right. \\ & \frac{11}{2} \hat{n} \times \vec{S}_1 \cdot \vec{v}_1 \hat{n} \cdot \vec{v}_2 \hat{n} \cdot \vec{v}_1 - \frac{9}{10} \vec{S}_1 \times \vec{v}_1 \cdot \vec{v}_2 \log\left(\frac{r}{R_\theta}\right) \hat{n} \cdot \vec{v}_1 + \frac{9}{2} \hat{n} \times \vec{S}_1 \cdot \vec{v}_1 \hat{n} \cdot \vec{v}_2 \log\left(\frac{r}{R_\theta}\right) \hat{n} \cdot \vec{v}_1 + \\ & 31 \hat{n} \times \vec{S}_1 \cdot \vec{v}_1 (\hat{n} \cdot \vec{v}_2)^2 - 10 \vec{S}_1 \times \vec{v}_1 \cdot \vec{v}_2 \hat{n} \cdot \vec{v}_2 + \frac{307}{350} \hat{n} \times \vec{S}_1 \cdot \vec{v}_1 \vec{v}_1 \cdot \vec{v}_1 + \frac{23}{25} \hat{n} \times \vec{S}_1 \cdot \vec{v}_1 \vec{v}_1 \cdot \vec{v}_2 - \\ & 5 \hat{n} \times \vec{S}_1 \cdot \vec{v}_1 \vec{v}_2 \cdot \vec{v}_2 - 30 \hat{n} \times \vec{S}_1 \cdot \vec{v}_1 (\hat{n} \cdot \vec{v}_2)^2 \log\left(\frac{r}{R_\theta}\right) + 12 \vec{S}_1 \times \vec{v}_1 \cdot \vec{v}_2 \hat{n} \cdot \vec{v}_2 \log\left(\frac{r}{R_\theta}\right) - \\ & \left. \frac{9}{10} \hat{n} \times \vec{S}_1 \cdot \vec{v}_1 \vec{v}_1 \cdot \vec{v}_1 \log\left(\frac{r}{R_\theta}\right) - \frac{9}{10} \hat{n} \times \vec{S}_1 \cdot \vec{v}_1 \vec{v}_1 \cdot \vec{v}_2 \log\left(\frac{r}{R_\theta}\right) + 6 \hat{n} \times \vec{S}_1 \cdot \vec{v}_1 \vec{v}_2 \cdot \vec{v}_2 \log\left(\frac{r}{R_\theta}\right) + \frac{1}{\epsilon_d} \right) \end{aligned}$$

$$\left( -\frac{3}{2} \hat{n} \times \vec{S}_1 \cdot \vec{v}_1 (\hat{n} \cdot \vec{v}_1)^2 + \frac{3}{10} \vec{S}_1 \times \vec{v}_1 \cdot \vec{v}_2 \hat{n} \cdot \vec{v}_1 - \frac{3}{2} \hat{n} \times \vec{S}_1 \cdot \vec{v}_1 \hat{n} \cdot \vec{v}_2 \hat{n} \cdot \vec{v}_1 + 10 \hat{n} \times \vec{S}_1 \cdot \vec{v}_1 (\hat{n} \cdot \vec{v}_2)^2 - \right. \\ \left. 4 \vec{S}_1 \times \vec{v}_1 \cdot \vec{v}_2 \hat{n} \cdot \vec{v}_2 + \frac{3}{10} \hat{n} \times \vec{S}_1 \cdot \vec{v}_1 \vec{v}_1 \cdot \vec{v}_1 + \frac{3}{10} \hat{n} \times \vec{S}_1 \cdot \vec{v}_1 \vec{v}_1 \cdot \vec{v}_2 - 2 \hat{n} \times \vec{S}_1 \cdot \vec{v}_1 \vec{v}_2 \cdot \vec{v}_2 \right) G^3 \}$$

$$\{ \text{DiagSet}[3, 1, 201], \text{Diagram} \},$$
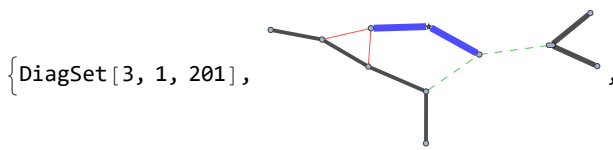

$$\frac{1}{r^3} G^3 m_2^3 \left( \frac{-\frac{2}{5} \hat{n} \cdot \vec{a}_2 \hat{n} \times \vec{S}_1 \cdot \vec{v}_2 - \frac{3}{5} \hat{n} \cdot \vec{v}_2 \hat{n} \times \vec{a}_2 \cdot \vec{S}_1 + \frac{1}{3} \vec{a}_2 \times \vec{S}_1 \cdot \vec{v}_2 + \frac{1}{5} \hat{n} \cdot \vec{v}_2 \hat{n} \times \vec{S}_1 \cdot \vec{v}_2}{\epsilon_d} + \right. \\ \frac{6}{5} \log\left(\frac{r}{R_\theta}\right) \hat{n} \cdot \vec{a}_2 \hat{n} \times \vec{S}_1 \cdot \vec{v}_2 + \frac{9}{5} \log\left(\frac{r}{R_\theta}\right) \hat{n} \cdot \vec{v}_2 \hat{n} \times \vec{a}_2 \cdot \vec{S}_1 - \frac{37}{75} \hat{n} \cdot \vec{a}_2 \hat{n} \times \vec{S}_1 \cdot \vec{v}_2 - \frac{46}{25} \hat{n} \cdot \vec{v}_2 \hat{n} \times \vec{a}_2 \cdot \vec{S}_1 - \\ \left. \log\left(\frac{r}{R_\theta}\right) \vec{a}_2 \times \vec{S}_1 \cdot \vec{v}_2 + \frac{4}{9} \vec{a}_2 \times \vec{S}_1 \cdot \vec{v}_2 - \frac{3}{5} \log\left(\frac{r}{R_\theta}\right) \hat{n} \cdot \vec{v}_2 \hat{n} \times \vec{S}_1 \cdot \vec{v}_2 + \frac{101}{75} \hat{n} \cdot \vec{v}_2 \hat{n} \times \vec{S}_1 \cdot \vec{v}_2 \right) + \frac{1}{r^4} G^3 m_2^3 \\ \left( \frac{1}{\epsilon_d} \left( \frac{8}{7} (\hat{n} \cdot \vec{v}_2)^2 \hat{n} \times \vec{S}_1 \cdot \vec{v}_2 - \frac{1}{5} \hat{n} \cdot \vec{v}_2 \vec{S}_1 \times \vec{v}_1 \cdot \vec{v}_2 - \hat{n} \cdot \vec{v}_1 \hat{n} \cdot \vec{v}_2 \hat{n} \times \vec{S}_1 \cdot \vec{v}_2 + \frac{1}{5} \vec{v}_1 \cdot \vec{v}_2 \hat{n} \times \vec{S}_1 \cdot \vec{v}_2 - \frac{8}{35} \vec{v}_2 \cdot \vec{v}_2 \hat{n} \times \vec{S}_1 \cdot \vec{v}_2 \right) - \right. \\ \frac{24}{7} \log\left(\frac{r}{R_\theta}\right) (\hat{n} \cdot \vec{v}_2)^2 \hat{n} \times \vec{S}_1 \cdot \vec{v}_2 + \frac{3}{5} \log\left(\frac{r}{R_\theta}\right) \hat{n} \cdot \vec{v}_2 \vec{S}_1 \times \vec{v}_1 \cdot \vec{v}_2 + 3 \log\left(\frac{r}{R_\theta}\right) \hat{n} \cdot \vec{v}_1 \hat{n} \cdot \vec{v}_2 \hat{n} \times \vec{S}_1 \cdot \vec{v}_2 - \\ \frac{3}{5} \log\left(\frac{r}{R_\theta}\right) \vec{v}_1 \cdot \vec{v}_2 \hat{n} \times \vec{S}_1 \cdot \vec{v}_2 + \frac{24}{35} \log\left(\frac{r}{R_\theta}\right) \vec{v}_2 \cdot \vec{v}_2 \hat{n} \times \vec{S}_1 \cdot \vec{v}_2 + \frac{859}{147} (\hat{n} \cdot \vec{v}_2)^2 \hat{n} \times \vec{S}_1 \cdot \vec{v}_2 - \\ \left. \frac{101}{75} \hat{n} \cdot \vec{v}_2 \vec{S}_1 \times \vec{v}_1 \cdot \vec{v}_2 - \frac{22}{3} \hat{n} \cdot \vec{v}_1 \hat{n} \cdot \vec{v}_2 \hat{n} \times \vec{S}_1 \cdot \vec{v}_2 + \frac{101}{75} \vec{v}_1 \cdot \vec{v}_2 \hat{n} \times \vec{S}_1 \cdot \vec{v}_2 - \frac{2951 \vec{v}_2 \cdot \vec{v}_2 \hat{n} \times \vec{S}_1 \cdot \vec{v}_2}{3675} \right) \}$$

$$\{ \text{DiagSet}[3, 1, 202], \text{Diagram} \}, -\frac{G^3 \hat{n} \times \vec{S}_1 \cdot \vec{v}_2 m_2^3}{9 r^2} + \frac{1}{r^3}$$
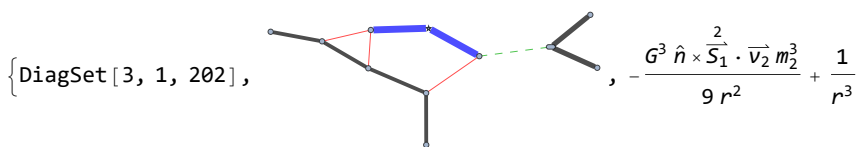

$$G^3 \left( \frac{2}{9} \frac{1}{\vec{S}_1 \times \vec{v}_1 \cdot \vec{v}_2} - \frac{1}{9} \vec{a}_1 \times \vec{S}_1 \cdot \vec{v}_2 + \frac{1}{9} \vec{a}_2 \times \vec{S}_1 \cdot \vec{v}_2 + \frac{1}{3} \hat{n} \times \vec{S}_1 \cdot \vec{v}_2 \hat{n} \cdot \vec{a}_1 - \frac{38}{75} \hat{n} \times \vec{S}_1 \cdot \vec{v}_2 \hat{n} \cdot \vec{a}_2 + \frac{2}{3} \hat{n} \times \vec{S}_1 \cdot \vec{v}_2 \hat{n} \cdot \vec{v}_1 - \right. \\ \frac{34}{25} \hat{n} \times \vec{S}_1 \cdot \vec{v}_2 \hat{n} \cdot \vec{v}_2 + \frac{13}{75} \hat{n} \times \vec{a}_2 \cdot \vec{S}_1 \hat{n} \cdot \vec{v}_2 + \frac{3}{10} \hat{n} \times \vec{S}_1 \cdot \vec{v}_2 \hat{n} \cdot \vec{a}_2 \log\left(\frac{r}{R_\theta}\right) + \frac{6}{5} \hat{n} \times \vec{S}_1 \cdot \vec{v}_2 \hat{n} \cdot \vec{v}_2 \log\left(\frac{r}{R_\theta}\right) - \\ \left. \frac{3}{10} \hat{n} \times \vec{a}_2 \cdot \vec{S}_1 \hat{n} \cdot \vec{v}_2 \log\left(\frac{r}{R_\theta}\right) + \frac{-\frac{1}{10} \hat{n} \times \vec{S}_1 \cdot \vec{v}_2 \hat{n} \cdot \vec{a}_2 - \frac{2}{5} \hat{n} \times \vec{S}_1 \cdot \vec{v}_2 \hat{n} \cdot \vec{v}_2 + \frac{1}{10} \hat{n} \times \vec{a}_2 \cdot \vec{S}_1 \hat{n} \cdot \vec{v}_2}{\epsilon_d} \right) m_2^3 + \frac{1}{r^4}$$

$$G^3 \left( -\frac{5}{3} \hat{n} \times \vec{S}_1 \cdot \vec{v}_2 (\hat{n} \cdot \vec{v}_1)^2 - \frac{2}{3} \vec{S}_1 \times \vec{v}_1 \cdot \vec{v}_2 \hat{n} \cdot \vec{v}_1 + 8 \hat{n} \times \vec{S}_1 \cdot \vec{v}_2 \hat{n} \cdot \vec{v}_2 \hat{n} \cdot \vec{v}_1 - 6 \hat{n} \times \vec{S}_1 \cdot \vec{v}_2 \hat{n} \cdot \vec{v}_2 \log\left(\frac{r}{R_\theta}\right) \hat{n} \cdot \vec{v}_1 - \right. \\ \frac{565}{147} \hat{n} \times \vec{S}_1 \cdot \vec{v}_2 (\hat{n} \cdot \vec{v}_2)^2 + \frac{34}{25} \vec{S}_1 \times \vec{v}_1 \cdot \vec{v}_2 \hat{n} \cdot \vec{v}_2 + \frac{1}{3} \hat{n} \times \vec{S}_1 \cdot \vec{v}_2 \vec{v}_1 \cdot \vec{v}_1 - \frac{34}{25} \hat{n} \times \vec{S}_1 \cdot \vec{v}_2 \vec{v}_1 \cdot \vec{v}_2 + \\ \frac{2951 \hat{n} \times \vec{S}_1 \cdot \vec{v}_2 \vec{v}_2 \cdot \vec{v}_2}{3675} + \frac{24}{7} \hat{n} \times \vec{S}_1 \cdot \vec{v}_2 (\hat{n} \cdot \vec{v}_2)^2 \log\left(\frac{r}{R_\theta}\right) - \frac{6}{5} \vec{S}_1 \times \vec{v}_1 \cdot \vec{v}_2 \hat{n} \cdot \vec{v}_2 \log\left(\frac{r}{R_\theta}\right) + \\ \left. \frac{6}{5} \hat{n} \times \vec{S}_1 \cdot \vec{v}_2 \vec{v}_1 \cdot \vec{v}_2 \log\left(\frac{r}{R_\theta}\right) - \frac{24}{35} \hat{n} \times \vec{S}_1 \cdot \vec{v}_2 \vec{v}_2 \cdot \vec{v}_2 \log\left(\frac{r}{R_\theta}\right) + \frac{1}{\epsilon_d} \left( -\frac{8}{7} \hat{n} \times \vec{S}_1 \cdot \vec{v}_2 (\hat{n} \cdot \vec{v}_2)^2 + \right. \right.$$



$$\left. \frac{2}{5} \vec{S}_1 \times \vec{v}_1 \cdot \vec{v}_2 \hat{n} \cdot \vec{v}_2 + 2 \hat{n} \times \vec{S}_1 \cdot \vec{v}_2 \hat{n} \cdot \vec{v}_1 \hat{n} \cdot \vec{v}_2 - \frac{2}{5} \hat{n} \times \vec{S}_1 \cdot \vec{v}_2 \vec{v}_1 \cdot \vec{v}_2 + \frac{8}{35} \hat{n} \times \vec{S}_1 \cdot \vec{v}_2 \vec{v}_2 \cdot \vec{v}_2 \right) m_2^3 \Bigg\}$$

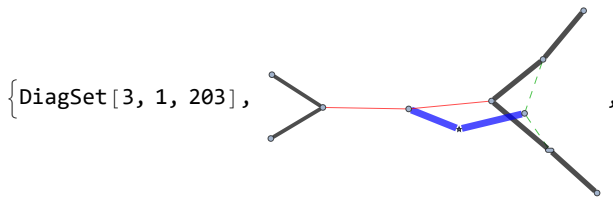

$$\begin{aligned} & \frac{1}{r^3} m_1^2 m_2 \left( -2 \log \left( \frac{r}{R_\theta} \right) \frac{1}{\vec{S}_1 \times \vec{v}_1 \cdot \vec{v}_2} + \frac{14}{9} \frac{1}{\vec{S}_1 \times \vec{v}_1 \cdot \vec{v}_2} + \frac{14}{9} \vec{S}_1 \times \vec{a}_1 \cdot \vec{v}_2 + \frac{89}{225} \vec{S}_1 \times \vec{v}_1 \cdot \vec{a}_1 + \right. \\ & \frac{58}{25} \hat{n} \times \vec{S}_1 \cdot \vec{v}_1 \hat{n} \cdot \vec{a}_1 + \frac{482}{75} \hat{n} \times \vec{S}_1 \cdot \vec{v}_1 \hat{n} \cdot \vec{v}_1 + \frac{308}{75} \hat{n} \times \vec{S}_1 \cdot \vec{a}_1 \hat{n} \cdot \vec{v}_1 - \frac{20}{3} \hat{n} \times \vec{S}_1 \cdot \vec{v}_1 \hat{n} \cdot \vec{v}_2 - \\ & \frac{20}{3} \hat{n} \times \vec{S}_1 \cdot \vec{a}_1 \hat{n} \cdot \vec{v}_2 - 2 \vec{S}_1 \times \vec{a}_1 \cdot \vec{v}_2 \log \left( \frac{r}{R_\theta} \right) - \frac{4}{5} \vec{S}_1 \times \vec{v}_1 \cdot \vec{a}_1 \log \left( \frac{r}{R_\theta} \right) - \frac{12}{5} \hat{n} \times \vec{S}_1 \cdot \vec{v}_1 \hat{n} \cdot \vec{a}_1 \log \left( \frac{r}{R_\theta} \right) - \\ & \frac{36}{5} \hat{n} \times \vec{S}_1 \cdot \vec{v}_1 \hat{n} \cdot \vec{v}_1 \log \left( \frac{r}{R_\theta} \right) - \frac{24}{5} \hat{n} \times \vec{S}_1 \cdot \vec{a}_1 \hat{n} \cdot \vec{v}_1 \log \left( \frac{r}{R_\theta} \right) + 6 \hat{n} \times \vec{S}_1 \cdot \vec{v}_1 \hat{n} \cdot \vec{v}_2 \log \left( \frac{r}{R_\theta} \right) + \\ & 6 \hat{n} \times \vec{S}_1 \cdot \vec{a}_1 \hat{n} \cdot \vec{v}_2 \log \left( \frac{r}{R_\theta} \right) + \frac{1}{\epsilon_d} \left( \frac{2}{3} \frac{1}{\vec{S}_1 \times \vec{v}_1 \cdot \vec{v}_2} + \frac{2}{3} \vec{S}_1 \times \vec{a}_1 \cdot \vec{v}_2 + \frac{4}{15} \vec{S}_1 \times \vec{v}_1 \cdot \vec{a}_1 + \frac{4}{5} \hat{n} \times \vec{S}_1 \cdot \vec{v}_1 \hat{n} \cdot \vec{a}_1 + \right. \\ & \left. \frac{12}{5} \hat{n} \times \vec{S}_1 \cdot \vec{v}_1 \hat{n} \cdot \vec{v}_1 + \frac{8}{5} \hat{n} \times \vec{S}_1 \cdot \vec{a}_1 \hat{n} \cdot \vec{v}_1 - 2 \hat{n} \times \vec{S}_1 \cdot \vec{v}_1 \hat{n} \cdot \vec{v}_2 - 2 \hat{n} \times \vec{S}_1 \cdot \vec{a}_1 \hat{n} \cdot \vec{v}_2 \right) \Bigg) G^3 + \\ & \frac{1}{r^4} m_1^2 m_2 \left( -\frac{386}{147} \hat{n} \times \vec{S}_1 \cdot \vec{v}_1 (\hat{n} \cdot \vec{v}_1)^2 - \frac{12}{7} \hat{n} \times \vec{S}_1 \cdot \vec{v}_1 \log \left( \frac{r}{R_\theta} \right) (\hat{n} \cdot \vec{v}_1)^2 - \frac{6}{25} \vec{S}_1 \times \vec{v}_1 \cdot \vec{v}_2 \hat{n} \cdot \vec{v}_1 - \right. \\ & \frac{6}{5} \vec{S}_1 \times \vec{v}_1 \cdot \vec{v}_2 \log \left( \frac{r}{R_\theta} \right) \hat{n} \cdot \vec{v}_1 + 6 \hat{n} \times \vec{S}_1 \cdot \vec{v}_1 \hat{n} \cdot \vec{v}_2 \log \left( \frac{r}{R_\theta} \right) \hat{n} \cdot \vec{v}_1 - \frac{1808 \hat{n} \times \vec{S}_1 \cdot \vec{v}_1 \vec{v}_1 \cdot \vec{v}_1}{3675} - \frac{6}{25} \hat{n} \times \vec{S}_1 \cdot \vec{v}_1 \vec{v}_1 \cdot \vec{v}_2 + \\ & \frac{12}{35} \hat{n} \times \vec{S}_1 \cdot \vec{v}_1 \vec{v}_1 \cdot \vec{v}_1 \log \left( \frac{r}{R_\theta} \right) - \frac{6}{5} \hat{n} \times \vec{S}_1 \cdot \vec{v}_1 \vec{v}_1 \cdot \vec{v}_2 \log \left( \frac{r}{R_\theta} \right) + \frac{1}{\epsilon_d} \left( \frac{4}{7} \hat{n} \times \vec{S}_1 \cdot \vec{v}_1 (\hat{n} \cdot \vec{v}_1)^2 + \right. \\ & \left. \frac{2}{5} \vec{S}_1 \times \vec{v}_1 \cdot \vec{v}_2 \hat{n} \cdot \vec{v}_1 - 2 \hat{n} \times \vec{S}_1 \cdot \vec{v}_1 \hat{n} \cdot \vec{v}_2 \hat{n} \cdot \vec{v}_1 - \frac{4}{35} \hat{n} \times \vec{S}_1 \cdot \vec{v}_1 \vec{v}_1 \cdot \vec{v}_1 + \frac{2}{5} \hat{n} \times \vec{S}_1 \cdot \vec{v}_1 \vec{v}_1 \cdot \vec{v}_2 \right) \Bigg) G^3 \Bigg\} \end{aligned}$$

{DiagSet[3, 1, 204], 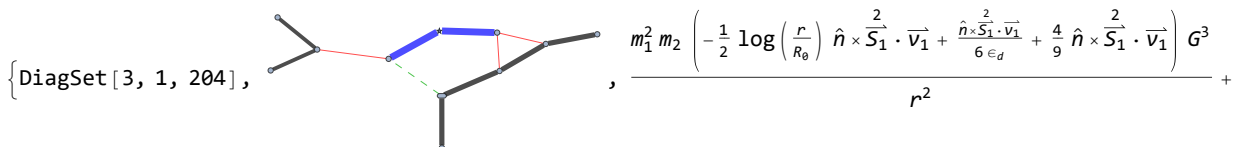 ,  $\frac{m_1^2 m_2 \left( -\frac{1}{2} \log \left( \frac{r}{R_\theta} \right) \hat{n} \times \vec{S}_1 \cdot \vec{v}_1 + \frac{\hat{n} \times \vec{S}_1 \cdot \vec{v}_1}{6 \epsilon_d} + \frac{4}{9} \hat{n} \times \vec{S}_1 \cdot \vec{v}_1 \right) G^3}{r^2} +$

$$\begin{aligned} & \frac{1}{r^3} m_1^2 m_2 \left( \log \left( \frac{r}{R_\theta} \right) \frac{1}{\vec{S}_1 \times \vec{v}_1 \cdot \vec{v}_2} - \frac{8}{9} \frac{1}{\vec{S}_1 \times \vec{v}_1 \cdot \vec{v}_2} + \frac{4}{9} \vec{S}_1 \times \vec{v}_1 \cdot \vec{a}_1 - \frac{4}{9} \vec{S}_1 \times \vec{v}_1 \cdot \vec{a}_2 - \frac{199}{150} \hat{n} \times \vec{S}_1 \cdot \vec{v}_1 \hat{n} \cdot \vec{a}_1 + \right. \\ & \frac{11}{6} \hat{n} \times \vec{S}_1 \cdot \vec{v}_1 \hat{n} \cdot \vec{a}_2 - \frac{41}{25} \hat{n} \times \vec{S}_1 \cdot \vec{v}_1 \hat{n} \cdot \vec{v}_1 + \frac{38}{75} \hat{n} \times \vec{S}_1 \cdot \vec{a}_1 \hat{n} \cdot \vec{v}_1 + \frac{11}{3} \hat{n} \times \vec{S}_1 \cdot \vec{v}_1 \hat{n} \cdot \vec{v}_2 - \frac{1}{2} \vec{S}_1 \times \vec{v}_1 \cdot \vec{a}_1 \log \left( \frac{r}{R_\theta} \right) + \\ & \frac{1}{2} \vec{S}_1 \times \vec{v}_1 \cdot \vec{a}_2 \log \left( \frac{r}{R_\theta} \right) + \frac{6}{5} \hat{n} \times \vec{S}_1 \cdot \vec{v}_1 \hat{n} \cdot \vec{a}_1 \log \left( \frac{r}{R_\theta} \right) - \frac{3}{2} \hat{n} \times \vec{S}_1 \cdot \vec{v}_1 \hat{n} \cdot \vec{a}_2 \log \left( \frac{r}{R_\theta} \right) + \frac{9}{5} \hat{n} \times \vec{S}_1 \cdot \vec{v}_1 \hat{n} \cdot \vec{v}_1 \log \left( \frac{r}{R_\theta} \right) - \\ & \frac{3}{10} \hat{n} \times \vec{S}_1 \cdot \vec{a}_1 \hat{n} \cdot \vec{v}_1 \log \left( \frac{r}{R_\theta} \right) - 3 \hat{n} \times \vec{S}_1 \cdot \vec{v}_1 \hat{n} \cdot \vec{v}_2 \log \left( \frac{r}{R_\theta} \right) + \frac{1}{\epsilon_d} \left( -\frac{1}{3} \frac{1}{\vec{S}_1 \times \vec{v}_1 \cdot \vec{v}_2} + \frac{1}{6} \vec{S}_1 \times \vec{v}_1 \cdot \vec{a}_1 - \frac{1}{6} \vec{S}_1 \times \vec{v}_1 \cdot \vec{a}_2 - \right. \\ & \left. \frac{2}{5} \hat{n} \times \vec{S}_1 \cdot \vec{v}_1 \hat{n} \cdot \vec{a}_1 + \frac{1}{2} \hat{n} \times \vec{S}_1 \cdot \vec{v}_1 \hat{n} \cdot \vec{a}_2 - \frac{3}{5} \hat{n} \times \vec{S}_1 \cdot \vec{v}_1 \hat{n} \cdot \vec{v}_1 + \frac{1}{10} \hat{n} \times \vec{S}_1 \cdot \vec{a}_1 \hat{n} \cdot \vec{v}_1 + \hat{n} \times \vec{S}_1 \cdot \vec{v}_1 \hat{n} \cdot \vec{v}_2 \right) \Bigg) G^3 + \frac{1}{r^4} \\ & m_1^2 m_2 \left( \frac{562}{147} \hat{n} \times \vec{S}_1 \cdot \vec{v}_1 (\hat{n} \cdot \vec{v}_1)^2 - \frac{57}{14} \hat{n} \times \vec{S}_1 \cdot \vec{v}_1 \log \left( \frac{r}{R_\theta} \right) (\hat{n} \cdot \vec{v}_1)^2 + \frac{41}{25} \vec{S}_1 \times \vec{v}_1 \cdot \vec{v}_2 \hat{n} \cdot \vec{v}_1 - 10 \hat{n} \times \vec{S}_1 \cdot \vec{v}_1 \hat{n} \cdot \vec{v}_2 \hat{n} \cdot \vec{v}_1 - \right. \\ & \left. \frac{9}{5} \vec{S}_1 \times \vec{v}_1 \cdot \vec{v}_2 \log \left( \frac{r}{R_\theta} \right) \hat{n} \cdot \vec{v}_1 + 9 \hat{n} \times \vec{S}_1 \cdot \vec{v}_1 \hat{n} \cdot \vec{v}_2 \log \left( \frac{r}{R_\theta} \right) \hat{n} \cdot \vec{v}_1 + \frac{32}{3} \hat{n} \times \vec{S}_1 \cdot \vec{v}_1 (\hat{n} \cdot \vec{v}_2)^2 - \frac{11}{3} \vec{S}_1 \times \vec{v}_1 \cdot \vec{v}_2 \hat{n} \cdot \vec{v}_2 - \right. \end{aligned}$$

$$\frac{7573 \hat{n} \times \vec{S}_1 \cdot \vec{v}_1 \vec{v}_1 \cdot \vec{v}_1}{7350} + \frac{41}{25} \hat{n} \times \vec{S}_1 \cdot \vec{v}_1 \vec{v}_1 \cdot \vec{v}_2 - \frac{11}{6} \hat{n} \times \vec{S}_1 \cdot \vec{v}_1 \vec{v}_2 \cdot \vec{v}_2 - \frac{15}{2} \hat{n} \times \vec{S}_1 \cdot \vec{v}_1 (\hat{n} \cdot \vec{v}_2)^2 \log\left(\frac{r}{R_0}\right) +$$

$$3 \vec{S}_1 \times \vec{v}_1 \cdot \vec{v}_2 \hat{n} \cdot \vec{v}_2 \log\left(\frac{r}{R_0}\right) + \frac{57}{70} \hat{n} \times \vec{S}_1 \cdot \vec{v}_1 \vec{v}_1 \cdot \vec{v}_1 \log\left(\frac{r}{R_0}\right) - \frac{9}{5} \hat{n} \times \vec{S}_1 \cdot \vec{v}_1 \vec{v}_1 \cdot \vec{v}_2 \log\left(\frac{r}{R_0}\right) +$$

$$\frac{3}{2} \hat{n} \times \vec{S}_1 \cdot \vec{v}_1 \vec{v}_2 \cdot \vec{v}_2 \log\left(\frac{r}{R_0}\right) + \frac{1}{\epsilon_d} \left( \frac{19}{14} \hat{n} \times \vec{S}_1 \cdot \vec{v}_1 (\hat{n} \cdot \vec{v}_1)^2 + \frac{3}{5} \vec{S}_1 \times \vec{v}_1 \cdot \vec{v}_2 \hat{n} \cdot \vec{v}_1 - 3 \hat{n} \times \vec{S}_1 \cdot \vec{v}_1 \hat{n} \cdot \vec{v}_2 \hat{n} \cdot \vec{v}_1 + \right.$$

$$\left. \frac{5}{2} \hat{n} \times \vec{S}_1 \cdot \vec{v}_1 (\hat{n} \cdot \vec{v}_2)^2 - \vec{S}_1 \times \vec{v}_1 \cdot \vec{v}_2 \hat{n} \cdot \vec{v}_2 - \frac{19}{70} \hat{n} \times \vec{S}_1 \cdot \vec{v}_1 \vec{v}_1 \cdot \vec{v}_1 + \frac{3}{5} \hat{n} \times \vec{S}_1 \cdot \vec{v}_1 \vec{v}_1 \cdot \vec{v}_2 - \frac{1}{2} \hat{n} \times \vec{S}_1 \cdot \vec{v}_1 \vec{v}_2 \cdot \vec{v}_2 \right) \Bigg\} G^3 \Bigg\}$$

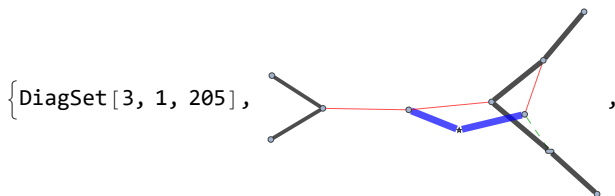

$$\frac{1}{r^3} G^3 m_1^2 m_2 \left( \frac{1}{\epsilon_d} \left( -\frac{3}{2} \hat{n} \cdot \vec{v}_1 \hat{n} \times \vec{S}_1 \cdot \vec{a}_1 + \frac{3}{2} \hat{n} \cdot \vec{v}_2 \hat{n} \times \vec{S}_1 \cdot \vec{a}_1 - \frac{1}{2} \vec{S}_1 \times \vec{a}_1 \cdot \vec{v}_2 - \frac{1}{2} \vec{S}_1 \times \vec{v}_1 \cdot \vec{a}_1 - \right. \right.$$

$$\left. \hat{n} \cdot \vec{v}_1 \hat{n} \times \vec{S}_1 \cdot \vec{v}_1 + \hat{n} \cdot \vec{v}_2 \hat{n} \times \vec{S}_1 \cdot \vec{v}_1 - \frac{1}{3} \vec{S}_1 \times \vec{v}_1 \cdot \vec{v}_2 \right) + \frac{9}{2} \log\left(\frac{r}{R_0}\right) \hat{n} \cdot \vec{v}_1 \hat{n} \times \vec{S}_1 \cdot \vec{a}_1 -$$

$$\frac{9}{2} \log\left(\frac{r}{R_0}\right) \hat{n} \cdot \vec{v}_2 \hat{n} \times \vec{S}_1 \cdot \vec{a}_1 - \frac{7}{2} \hat{n} \cdot \vec{v}_1 \hat{n} \times \vec{S}_1 \cdot \vec{a}_1 + \frac{9}{2} \hat{n} \cdot \vec{v}_2 \hat{n} \times \vec{S}_1 \cdot \vec{a}_1 + \frac{3}{2} \log\left(\frac{r}{R_0}\right) \vec{S}_1 \times \vec{a}_1 \cdot \vec{v}_2 +$$

$$\frac{3}{2} \log\left(\frac{r}{R_0}\right) \vec{S}_1 \times \vec{v}_1 \cdot \vec{a}_1 - \vec{S}_1 \times \vec{a}_1 \cdot \vec{v}_2 - \vec{S}_1 \times \vec{v}_1 \cdot \vec{a}_1 + 3 \log\left(\frac{r}{R_0}\right) \hat{n} \cdot \vec{v}_1 \hat{n} \times \vec{S}_1 \cdot \vec{v}_1 -$$

$$3 \log\left(\frac{r}{R_0}\right) \hat{n} \cdot \vec{v}_2 \hat{n} \times \vec{S}_1 \cdot \vec{v}_1 - 2 \hat{n} \cdot \vec{v}_1 \hat{n} \times \vec{S}_1 \cdot \vec{v}_1 + \frac{7}{3} \hat{n} \cdot \vec{v}_2 \hat{n} \times \vec{S}_1 \cdot \vec{v}_1 + \log\left(\frac{r}{R_0}\right) \vec{S}_1 \times \vec{v}_1 \cdot \vec{v}_2 - \frac{4}{9} \vec{S}_1 \times \vec{v}_1 \cdot \vec{v}_2 \Bigg) +$$

$$\frac{G^3 m_1^2 m_2 \left( \frac{\hat{n} \times \vec{S}_1 \cdot \vec{v}_1}{6 \epsilon_d} - \frac{1}{2} \log\left(\frac{r}{R_0}\right) \hat{n} \times \vec{S}_1 \cdot \vec{v}_1 + \frac{5}{9} \hat{n} \times \vec{S}_1 \cdot \vec{v}_1 \right)}{r^2} + \frac{1}{r^4}$$

$$G^3 m_1^2 m_2 \left( 3 (\hat{n} \cdot \vec{v}_1)^2 \hat{n} \times \vec{S}_1 \cdot \vec{v}_1 + \hat{n} \cdot \vec{v}_1 \vec{S}_1 \times \vec{v}_1 \cdot \vec{v}_2 - 5 \hat{n} \cdot \vec{v}_2 \hat{n} \cdot \vec{v}_1 \hat{n} \times \vec{S}_1 \cdot \vec{v}_1 + \vec{v}_1 \cdot \vec{v}_2 \hat{n} \times \vec{S}_1 \cdot \vec{v}_1 \right) \Bigg\}$$

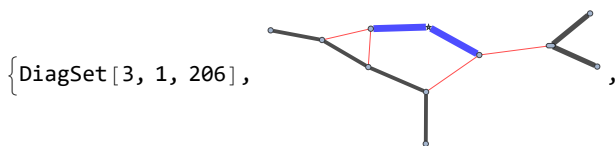

$$G^3 m_2^3 \left( -\frac{2}{3} \hat{n} \cdot \vec{v}_2 \hat{n} \times \vec{a}_1 \cdot \vec{S}_1 + \frac{2}{9} \vec{a}_1 \times \vec{S}_1 \cdot \vec{v}_2 + \frac{2}{3} \hat{n} \cdot \vec{v}_2 \hat{n} \times \vec{S}_1 \cdot \vec{v}_1 - \frac{2}{9} \vec{S}_1 \times \vec{v}_1 \cdot \vec{v}_2 \right) \frac{1}{r^3} + \frac{1}{r^4}$$

$$G^3 m_2^3 \left( \frac{(\hat{n} \cdot \vec{v}_2)^2 \left( -(\hat{n} \times \vec{S}_1 \cdot \vec{v}_1) \right) + \frac{2}{5} \hat{n} \cdot \vec{v}_2 \vec{S}_1 \times \vec{v}_1 \cdot \vec{v}_2 + \frac{1}{5} \vec{v}_2 \cdot \vec{v}_2 \hat{n} \times \vec{S}_1 \cdot \vec{v}_1}{\epsilon_d} + 3 \log\left(\frac{r}{R_0}\right) (\hat{n} \cdot \vec{v}_2)^2 \hat{n} \times \vec{S}_1 \cdot \vec{v}_1 - \right.$$

$$\frac{6}{5} \log\left(\frac{r}{R_0}\right) \hat{n} \cdot \vec{v}_2 \vec{S}_1 \times \vec{v}_1 \cdot \vec{v}_2 - \frac{3}{5} \log\left(\frac{r}{R_0}\right) \vec{v}_2 \cdot \vec{v}_2 \hat{n} \times \vec{S}_1 \cdot \vec{v}_1 - \frac{5}{3} (\hat{n} \cdot \vec{v}_2)^2 \hat{n} \times \vec{S}_1 \cdot \vec{v}_1 + \frac{32}{75} \hat{n} \cdot \vec{v}_2 \vec{S}_1 \times \vec{v}_1 \cdot \vec{v}_2 -$$

$$\left. \frac{10}{3} \hat{n} \cdot \vec{v}_1 \hat{n} \cdot \vec{v}_2 \hat{n} \times \vec{S}_1 \cdot \vec{v}_1 + \frac{2}{3} \hat{n} \cdot \vec{v}_1 \vec{S}_1 \times \vec{v}_1 \cdot \vec{v}_2 + \frac{2}{3} \vec{v}_1 \cdot \vec{v}_2 \hat{n} \times \vec{S}_1 \cdot \vec{v}_1 + \frac{76}{75} \vec{v}_2 \cdot \vec{v}_2 \hat{n} \times \vec{S}_1 \cdot \vec{v}_1 \right) \Bigg\}$$

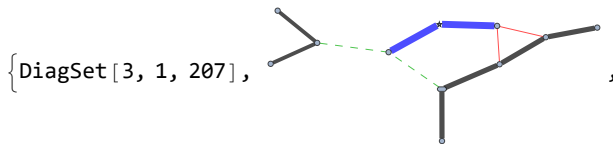

$$\begin{aligned} & \frac{1}{r^3} m_1^2 m_2 \left( -\frac{1}{5} \log\left(\frac{r}{R_0}\right) \frac{1}{\vec{S}_1 \times \vec{v}_1 \cdot \vec{v}_2} - \frac{19}{225} \frac{1}{\vec{S}_1 \times \vec{v}_1 \cdot \vec{v}_2} - \frac{19}{225} \vec{S}_1 \times \vec{v}_1 \cdot \vec{a}_2 - \frac{77}{75} \hat{n} \times \vec{S}_1 \cdot \vec{v}_1 \hat{n} \cdot \vec{a}_2 - \frac{22}{25} \hat{n} \times \vec{S}_1 \cdot \vec{v}_2 \hat{n} \cdot \vec{v}_1 - \right. \\ & \frac{22}{25} \hat{n} \times \vec{S}_1 \cdot \vec{a}_2 \hat{n} \cdot \vec{v}_1 - \frac{77}{75} \hat{n} \times \vec{S}_1 \cdot \vec{v}_1 \hat{n} \cdot \vec{v}_2 - \frac{1}{5} \vec{S}_1 \times \vec{v}_1 \cdot \vec{a}_2 \log\left(\frac{r}{R_0}\right) + \frac{6}{5} \hat{n} \times \vec{S}_1 \cdot \vec{v}_1 \hat{n} \cdot \vec{a}_2 \log\left(\frac{r}{R_0}\right) + \\ & \frac{3}{5} \hat{n} \times \vec{S}_1 \cdot \vec{v}_2 \hat{n} \cdot \vec{v}_1 \log\left(\frac{r}{R_0}\right) + \frac{3}{5} \hat{n} \times \vec{S}_1 \cdot \vec{a}_2 \hat{n} \cdot \vec{v}_1 \log\left(\frac{r}{R_0}\right) + \frac{6}{5} \hat{n} \times \vec{S}_1 \cdot \vec{v}_1 \hat{n} \cdot \vec{v}_2 \log\left(\frac{r}{R_0}\right) + \frac{1}{\epsilon_d} \\ & \left. \left( \frac{1}{15} \frac{1}{\vec{S}_1 \times \vec{v}_1 \cdot \vec{v}_2} + \frac{1}{15} \vec{S}_1 \times \vec{v}_1 \cdot \vec{a}_2 - \frac{2}{5} \hat{n} \times \vec{S}_1 \cdot \vec{v}_1 \hat{n} \cdot \vec{a}_2 - \frac{1}{5} \hat{n} \times \vec{S}_1 \cdot \vec{v}_2 \hat{n} \cdot \vec{v}_1 - \frac{1}{5} \hat{n} \times \vec{S}_1 \cdot \vec{a}_2 \hat{n} \cdot \vec{v}_1 - \frac{2}{5} \hat{n} \times \vec{S}_1 \cdot \vec{v}_1 \hat{n} \cdot \vec{v}_2 \right) \right) \\ & G^3 + \frac{1}{r^4} m_1^2 m_2 \left( \frac{628}{147} \hat{n} \times \vec{S}_1 \cdot \vec{v}_2 (\hat{n} \cdot \vec{v}_1)^2 - \frac{24}{7} \hat{n} \times \vec{S}_1 \cdot \vec{v}_2 \log\left(\frac{r}{R_0}\right) (\hat{n} \cdot \vec{v}_1)^2 + \frac{1948 \vec{S}_1 \times \vec{v}_1 \cdot \vec{v}_2 \hat{n} \cdot \vec{v}_1}{1225} + \right. \\ & \frac{125}{147} \hat{n} \times \vec{S}_1 \cdot \vec{v}_1 \hat{n} \cdot \vec{v}_2 \hat{n} \cdot \vec{v}_1 - 5 \hat{n} \times \vec{S}_1 \cdot \vec{v}_2 \hat{n} \cdot \vec{v}_2 \hat{n} \cdot \vec{v}_1 - \frac{36}{35} \vec{S}_1 \times \vec{v}_1 \cdot \vec{v}_2 \log\left(\frac{r}{R_0}\right) \hat{n} \cdot \vec{v}_1 - \\ & \frac{12}{7} \hat{n} \times \vec{S}_1 \cdot \vec{v}_1 \hat{n} \cdot \vec{v}_2 \log\left(\frac{r}{R_0}\right) \hat{n} \cdot \vec{v}_1 + 3 \hat{n} \times \vec{S}_1 \cdot \vec{v}_2 \hat{n} \cdot \vec{v}_2 \log\left(\frac{r}{R_0}\right) \hat{n} \cdot \vec{v}_1 - \frac{19}{3} \hat{n} \times \vec{S}_1 \cdot \vec{v}_1 (\hat{n} \cdot \vec{v}_2)^2 + \\ & \frac{73}{75} \vec{S}_1 \times \vec{v}_1 \cdot \vec{v}_2 \hat{n} \cdot \vec{v}_2 - \frac{3266 \hat{n} \times \vec{S}_1 \cdot \vec{v}_2 \vec{v}_1 \cdot \vec{v}_1}{3675} + \frac{47 \hat{n} \times \vec{S}_1 \cdot \vec{v}_1 \vec{v}_1 \cdot \vec{v}_2}{3675} + \frac{22}{25} \hat{n} \times \vec{S}_1 \cdot \vec{v}_2 \vec{v}_1 \cdot \vec{v}_2 + \\ & \frac{77}{75} \hat{n} \times \vec{S}_1 \cdot \vec{v}_1 \vec{v}_2 \cdot \vec{v}_2 + 6 \hat{n} \times \vec{S}_1 \cdot \vec{v}_1 (\hat{n} \cdot \vec{v}_2)^2 \log\left(\frac{r}{R_0}\right) - \frac{9}{5} \vec{S}_1 \times \vec{v}_1 \cdot \vec{v}_2 \hat{n} \cdot \vec{v}_2 \log\left(\frac{r}{R_0}\right) + \\ & \frac{24}{35} \hat{n} \times \vec{S}_1 \cdot \vec{v}_2 \vec{v}_1 \cdot \vec{v}_1 \log\left(\frac{r}{R_0}\right) + \frac{12}{35} \hat{n} \times \vec{S}_1 \cdot \vec{v}_1 \vec{v}_1 \cdot \vec{v}_2 \log\left(\frac{r}{R_0}\right) - \frac{3}{5} \hat{n} \times \vec{S}_1 \cdot \vec{v}_2 \vec{v}_1 \cdot \vec{v}_2 \log\left(\frac{r}{R_0}\right) - \\ & \frac{6}{5} \hat{n} \times \vec{S}_1 \cdot \vec{v}_1 \vec{v}_2 \cdot \vec{v}_2 \log\left(\frac{r}{R_0}\right) + \frac{1}{\epsilon_d} \left( \frac{8}{7} \hat{n} \times \vec{S}_1 \cdot \vec{v}_2 (\hat{n} \cdot \vec{v}_1)^2 + \frac{12}{35} \vec{S}_1 \times \vec{v}_1 \cdot \vec{v}_2 \hat{n} \cdot \vec{v}_1 + \right. \\ & \frac{4}{7} \hat{n} \times \vec{S}_1 \cdot \vec{v}_1 \hat{n} \cdot \vec{v}_2 \hat{n} \cdot \vec{v}_1 - \hat{n} \times \vec{S}_1 \cdot \vec{v}_2 \hat{n} \cdot \vec{v}_2 \hat{n} \cdot \vec{v}_1 - 2 \hat{n} \times \vec{S}_1 \cdot \vec{v}_1 (\hat{n} \cdot \vec{v}_2)^2 + \frac{3}{5} \vec{S}_1 \times \vec{v}_1 \cdot \vec{v}_2 \hat{n} \cdot \vec{v}_2 - \\ & \left. \left. \frac{8}{35} \hat{n} \times \vec{S}_1 \cdot \vec{v}_2 \vec{v}_1 \cdot \vec{v}_1 - \frac{4}{35} \hat{n} \times \vec{S}_1 \cdot \vec{v}_1 \vec{v}_1 \cdot \vec{v}_2 + \frac{1}{5} \hat{n} \times \vec{S}_1 \cdot \vec{v}_2 \vec{v}_1 \cdot \vec{v}_2 + \frac{2}{5} \hat{n} \times \vec{S}_1 \cdot \vec{v}_1 \vec{v}_2 \cdot \vec{v}_2 \right) \right) G^3 \} \end{aligned}$$

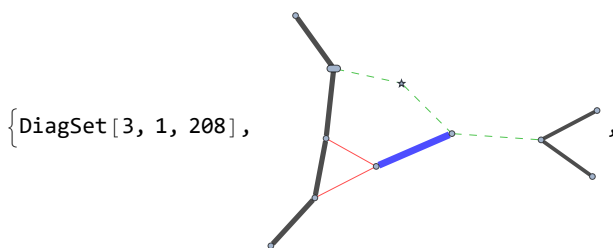

$$\begin{aligned} & \frac{m_1^2 m_2 \left( \hat{n} \times \vec{S}_1 \cdot \vec{a}_2 \log\left(\frac{r}{R_0}\right) - \frac{\hat{n} \times \vec{S}_1 \cdot \vec{a}_2}{3 \epsilon_d} \right) G^3}{r^2} + \frac{1}{r^3} m_1^2 m_2 \left( -\frac{3}{5} \log\left(\frac{r}{R_0}\right) \frac{1}{\vec{S}_1 \times \vec{v}_1 \cdot \vec{v}_2} - \frac{8}{25} \frac{1}{\vec{S}_1 \times \vec{v}_1 \cdot \vec{v}_2} + \frac{8}{25} \vec{S}_1 \times \vec{v}_1 \cdot \vec{a}_2 + \right. \\ & \frac{17}{25} \hat{n} \times \vec{S}_1 \cdot \vec{v}_1 \hat{n} \cdot \vec{a}_2 - \frac{11}{25} \hat{n} \times \vec{S}_1 \cdot \vec{v}_2 \hat{n} \cdot \vec{v}_1 + \frac{36}{25} \hat{n} \times \vec{S}_1 \cdot \vec{a}_2 \hat{n} \cdot \vec{v}_1 - \frac{17}{25} \hat{n} \times \vec{S}_1 \cdot \vec{v}_1 \hat{n} \cdot \vec{v}_2 - \hat{n} \times \vec{S}_1 \cdot \vec{v}_2 \hat{n} \cdot \vec{v}_2 - \\ & \frac{2}{5} \vec{S}_1 \times \vec{v}_1 \cdot \vec{a}_2 \log\left(\frac{r}{R_0}\right) - \frac{3}{5} \hat{n} \times \vec{S}_1 \cdot \vec{v}_1 \hat{n} \cdot \vec{a}_2 \log\left(\frac{r}{R_0}\right) - \frac{6}{5} \hat{n} \times \vec{S}_1 \cdot \vec{v}_2 \hat{n} \cdot \vec{v}_1 \log\left(\frac{r}{R_0}\right) - \frac{9}{5} \hat{n} \times \vec{S}_1 \cdot \vec{a}_2 \hat{n} \cdot \vec{v}_1 \log\left(\frac{r}{R_0}\right) + \\ & \left. \frac{3}{5} \hat{n} \times \vec{S}_1 \cdot \vec{v}_1 \hat{n} \cdot \vec{v}_2 \log\left(\frac{r}{R_0}\right) + 3 \hat{n} \times \vec{S}_1 \cdot \vec{v}_2 \hat{n} \cdot \vec{v}_2 \log\left(\frac{r}{R_0}\right) + \frac{1}{\epsilon_d} \left( \frac{1}{5} \vec{S}_1 \times \vec{v}_1 \cdot \vec{v}_2 + \frac{2}{15} \vec{S}_1 \times \vec{v}_1 \cdot \vec{a}_2 + \right. \right. \end{aligned}$$

$$\begin{aligned}
& \left. \frac{1}{5} \hat{n} \times \vec{S}_1 \cdot \vec{v}_1 \hat{n} \cdot \vec{a}_2 + \frac{2}{5} \hat{n} \times \vec{S}_1 \cdot \vec{v}_2 \hat{n} \cdot \vec{v}_1 + \frac{3}{5} \hat{n} \times \vec{S}_1 \cdot \vec{a}_2 \hat{n} \cdot \vec{v}_1 - \frac{1}{5} \hat{n} \times \vec{S}_1 \cdot \vec{v}_1 \hat{n} \cdot \vec{v}_2 - \hat{n} \times \vec{S}_1 \cdot \vec{v}_2 \hat{n} \cdot \vec{v}_2 \right) \left( G^3 + \frac{1}{r^4} \right. \\
& m_1^2 m_2 \left( -\frac{33}{49} \hat{n} \times \vec{S}_1 \cdot \vec{v}_2 (\hat{n} \cdot \vec{v}_1)^2 + \frac{9}{7} \hat{n} \times \vec{S}_1 \cdot \vec{v}_2 \log\left(\frac{r}{R_0}\right) (\hat{n} \cdot \vec{v}_1)^2 + \frac{456 \vec{S}_1 \times \vec{v}_1 \cdot \vec{v}_2 \hat{n} \cdot \vec{v}_1}{1225} - \frac{146}{49} \hat{n} \times \vec{S}_1 \cdot \vec{v}_1 \hat{n} \cdot \vec{v}_2 \hat{n} \cdot \vec{v}_1 + \right. \\
& 9 \hat{n} \times \vec{S}_1 \cdot \vec{v}_2 \hat{n} \cdot \vec{v}_2 \hat{n} \cdot \vec{v}_1 + \frac{3}{35} \vec{S}_1 \times \vec{v}_1 \cdot \vec{v}_2 \log\left(\frac{r}{R_0}\right) \hat{n} \cdot \vec{v}_1 + \frac{15}{7} \hat{n} \times \vec{S}_1 \cdot \vec{v}_1 \hat{n} \cdot \vec{v}_2 \log\left(\frac{r}{R_0}\right) \hat{n} \cdot \vec{v}_1 - \\
& 9 \hat{n} \times \vec{S}_1 \cdot \vec{v}_2 \hat{n} \cdot \vec{v}_2 \log\left(\frac{r}{R_0}\right) \hat{n} \cdot \vec{v}_1 + 4 \hat{n} \times \vec{S}_1 \cdot \vec{v}_1 (\hat{n} \cdot \vec{v}_2)^2 + \frac{17}{25} \vec{S}_1 \times \vec{v}_1 \cdot \vec{v}_2 \hat{n} \cdot \vec{v}_2 - \frac{248 \hat{n} \times \vec{S}_1 \cdot \vec{v}_2 \vec{v}_1 \cdot \vec{v}_1}{1225} + \\
& \frac{139}{245} \hat{n} \times \vec{S}_1 \cdot \vec{v}_1 \vec{v}_1 \cdot \vec{v}_2 - \frac{36}{25} \hat{n} \times \vec{S}_1 \cdot \vec{v}_2 \vec{v}_1 \cdot \vec{v}_2 - \frac{17}{25} \hat{n} \times \vec{S}_1 \cdot \vec{v}_1 \vec{v}_2 \cdot \vec{v}_2 - 3 \hat{n} \times \vec{S}_1 \cdot \vec{v}_1 (\hat{n} \cdot \vec{v}_2)^2 \log\left(\frac{r}{R_0}\right) - \\
& \frac{3}{5} \vec{S}_1 \times \vec{v}_1 \cdot \vec{v}_2 \hat{n} \cdot \vec{v}_2 \log\left(\frac{r}{R_0}\right) - \frac{9}{35} \hat{n} \times \vec{S}_1 \cdot \vec{v}_2 \vec{v}_1 \cdot \vec{v}_1 \log\left(\frac{r}{R_0}\right) - \frac{3}{7} \hat{n} \times \vec{S}_1 \cdot \vec{v}_1 \vec{v}_1 \cdot \vec{v}_2 \log\left(\frac{r}{R_0}\right) + \\
& \frac{9}{5} \hat{n} \times \vec{S}_1 \cdot \vec{v}_2 \vec{v}_1 \cdot \vec{v}_2 \log\left(\frac{r}{R_0}\right) + \frac{3}{5} \hat{n} \times \vec{S}_1 \cdot \vec{v}_1 \vec{v}_2 \cdot \vec{v}_2 \log\left(\frac{r}{R_0}\right) + \frac{1}{\epsilon_d} \left( -\frac{3}{7} \hat{n} \times \vec{S}_1 \cdot \vec{v}_2 (\hat{n} \cdot \vec{v}_1)^2 - \frac{1}{35} \vec{S}_1 \times \vec{v}_1 \cdot \vec{v}_2 \hat{n} \cdot \vec{v}_1 - \right. \\
& \frac{5}{7} \hat{n} \times \vec{S}_1 \cdot \vec{v}_1 \hat{n} \cdot \vec{v}_2 \hat{n} \cdot \vec{v}_1 + 3 \hat{n} \times \vec{S}_1 \cdot \vec{v}_2 \hat{n} \cdot \vec{v}_2 \hat{n} \cdot \vec{v}_1 + \hat{n} \times \vec{S}_1 \cdot \vec{v}_1 (\hat{n} \cdot \vec{v}_2)^2 + \frac{1}{5} \vec{S}_1 \times \vec{v}_1 \cdot \vec{v}_2 \hat{n} \cdot \vec{v}_2 + \\
& \left. \left. \frac{3}{35} \hat{n} \times \vec{S}_1 \cdot \vec{v}_2 \vec{v}_1 \cdot \vec{v}_1 + \frac{1}{7} \hat{n} \times \vec{S}_1 \cdot \vec{v}_1 \vec{v}_1 \cdot \vec{v}_2 - \frac{3}{5} \hat{n} \times \vec{S}_1 \cdot \vec{v}_2 \vec{v}_1 \cdot \vec{v}_2 - \frac{1}{5} \hat{n} \times \vec{S}_1 \cdot \vec{v}_1 \vec{v}_2 \cdot \vec{v}_2 \right) \right) G^3 \Big\}
\end{aligned}$$

{DiagSet[3, 1, 209],

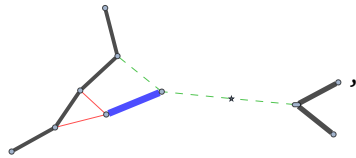

$$\begin{aligned}
& \frac{1}{r^3} G^3 m_2^3 \left( \frac{\frac{1}{5} \hat{n} \cdot \vec{v}_1 \hat{n} \times \vec{a}_2 \cdot \vec{S}_1 - \frac{1}{15} \vec{a}_2 \times \vec{S}_1 \cdot \vec{v}_1 + \frac{1}{5} \hat{n} \cdot \vec{v}_2 \hat{n} \times \vec{S}_1 \cdot \vec{v}_2}{\epsilon_d} - \frac{3}{5} \log\left(\frac{r}{R_0}\right) \hat{n} \cdot \vec{v}_1 \hat{n} \times \vec{a}_2 \cdot \vec{S}_1 + \frac{109}{50} \hat{n} \cdot \vec{v}_1 \hat{n} \times \vec{a}_2 \cdot \vec{S}_1 + \right. \\
& \left. \frac{1}{5} \log\left(\frac{r}{R_0}\right) \vec{a}_2 \times \vec{S}_1 \cdot \vec{v}_1 - \frac{33}{50} \vec{a}_2 \times \vec{S}_1 \cdot \vec{v}_1 - \frac{3}{5} \log\left(\frac{r}{R_0}\right) \hat{n} \cdot \vec{v}_2 \hat{n} \times \vec{S}_1 \cdot \vec{v}_2 + \frac{109}{50} \hat{n} \cdot \vec{v}_2 \hat{n} \times \vec{S}_1 \cdot \vec{v}_2 \right) + \\
& \frac{G^3 m_2^3 \left( -\frac{\hat{n} \times \vec{a}_2 \cdot \vec{S}_1}{15 \epsilon_d} + \frac{1}{5} \log\left(\frac{r}{R_0}\right) \hat{n} \times \vec{a}_2 \cdot \vec{S}_1 - \frac{33}{50} \hat{n} \times \vec{a}_2 \cdot \vec{S}_1 \right)}{r^2} + \frac{1}{r^4} \\
& G^3 m_2^3 \left( \frac{-\frac{1}{5} \hat{n} \cdot \vec{v}_2 \vec{S}_1 \times \vec{v}_1 \cdot \vec{v}_2 - \hat{n} \cdot \vec{v}_1 \hat{n} \cdot \vec{v}_2 \hat{n} \times \vec{S}_1 \cdot \vec{v}_2 + \frac{1}{5} \vec{v}_1 \cdot \vec{v}_2 \hat{n} \times \vec{S}_1 \cdot \vec{v}_2}{\epsilon_d} + \right. \\
& \frac{3}{5} \log\left(\frac{r}{R_0}\right) \hat{n} \cdot \vec{v}_2 \vec{S}_1 \times \vec{v}_1 \cdot \vec{v}_2 + 3 \log\left(\frac{r}{R_0}\right) \hat{n} \cdot \vec{v}_1 \hat{n} \cdot \vec{v}_2 \hat{n} \times \vec{S}_1 \cdot \vec{v}_2 - \frac{3}{5} \log\left(\frac{r}{R_0}\right) \vec{v}_1 \cdot \vec{v}_2 \hat{n} \times \vec{S}_1 \cdot \vec{v}_2 - \\
& \left. \frac{109}{50} \hat{n} \cdot \vec{v}_2 \vec{S}_1 \times \vec{v}_1 \cdot \vec{v}_2 - \frac{23}{2} \hat{n} \cdot \vec{v}_1 \hat{n} \cdot \vec{v}_2 \hat{n} \times \vec{S}_1 \cdot \vec{v}_2 + \frac{109}{50} \vec{v}_1 \cdot \vec{v}_2 \hat{n} \times \vec{S}_1 \cdot \vec{v}_2 \right) \Big\}
\end{aligned}$$

{DiagSet[3, 1, 210],

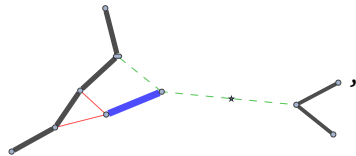

$$\frac{1}{r^3} G^3 m_1^2 m_2 \left( \frac{-\frac{1}{5} \hat{n} \cdot \vec{v}_1 \hat{n} \times \vec{S}_1 \cdot \vec{a}_2 - \frac{1}{15} \vec{S}_1 \times \vec{v}_1 \cdot \vec{a}_2 + \frac{1}{5} \hat{n} \cdot \vec{v}_2 \hat{n} \times \vec{S}_1 \cdot \vec{v}_2}{\epsilon_d} + \frac{3}{5} \log\left(\frac{r}{R_\theta}\right) \hat{n} \cdot \vec{v}_1 \hat{n} \times \vec{S}_1 \cdot \vec{a}_2 - \frac{49}{50} \hat{n} \cdot \vec{v}_1 \hat{n} \times \vec{S}_1 \cdot \vec{a}_2 + \right.$$

$$\left. \frac{1}{5} \log\left(\frac{r}{R_\theta}\right) \vec{S}_1 \times \vec{v}_1 \cdot \vec{a}_2 - \frac{13}{50} \vec{S}_1 \times \vec{v}_1 \cdot \vec{a}_2 - \frac{3}{5} \log\left(\frac{r}{R_\theta}\right) \hat{n} \cdot \vec{v}_2 \hat{n} \times \vec{S}_1 \cdot \vec{v}_2 + \frac{49}{50} \hat{n} \cdot \vec{v}_2 \hat{n} \times \vec{S}_1 \cdot \vec{v}_2 \right) +$$

$$\frac{G^3 m_1^2 m_2 \left( \frac{\hat{n} \times \vec{S}_1 \cdot \vec{a}_2}{15 \epsilon_d} - \frac{1}{5} \log\left(\frac{r}{R_\theta}\right) \hat{n} \times \vec{S}_1 \cdot \vec{a}_2 + \frac{13}{50} \hat{n} \times \vec{S}_1 \cdot \vec{a}_2 \right)}{r^2} + \frac{1}{r^4}$$

$$G^3 m_1^2 m_2 \left( \frac{-\frac{1}{5} \hat{n} \cdot \vec{v}_2 \vec{S}_1 \times \vec{v}_1 \cdot \vec{v}_2 - \hat{n} \cdot \vec{v}_1 \hat{n} \cdot \vec{v}_2 \hat{n} \times \vec{S}_1 \cdot \vec{v}_2 + \frac{1}{5} \vec{v}_1 \cdot \vec{v}_2 \hat{n} \times \vec{S}_1 \cdot \vec{v}_2}{\epsilon_d} + \right.$$

$$\left. \frac{3}{5} \log\left(\frac{r}{R_\theta}\right) \hat{n} \cdot \vec{v}_2 \vec{S}_1 \times \vec{v}_1 \cdot \vec{v}_2 + 3 \log\left(\frac{r}{R_\theta}\right) \hat{n} \cdot \vec{v}_1 \hat{n} \cdot \vec{v}_2 \hat{n} \times \vec{S}_1 \cdot \vec{v}_2 - \frac{3}{5} \log\left(\frac{r}{R_\theta}\right) \vec{v}_1 \cdot \vec{v}_2 \hat{n} \times \vec{S}_1 \cdot \vec{v}_2 - \right.$$

$$\left. \frac{49}{50} \hat{n} \cdot \vec{v}_2 \vec{S}_1 \times \vec{v}_1 \cdot \vec{v}_2 - \frac{11}{2} \hat{n} \cdot \vec{v}_1 \hat{n} \cdot \vec{v}_2 \hat{n} \times \vec{S}_1 \cdot \vec{v}_2 + \frac{49}{50} \vec{v}_1 \cdot \vec{v}_2 \hat{n} \times \vec{S}_1 \cdot \vec{v}_2 \right\}$$

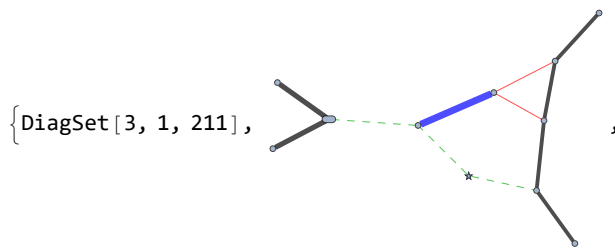

$$\frac{G^3 \hat{n} \times \vec{a}_2 \cdot \vec{S}_1 m_2^3}{3 r^2} + \frac{1}{r^3} G^3 \left( \frac{1}{3} \vec{a}_2 \times \vec{S}_1 \cdot \vec{v}_1 - \frac{1}{3} \vec{a}_2 \times \vec{S}_1 \cdot \vec{v}_2 + \frac{1}{25} \hat{n} \times \vec{S}_1 \cdot \vec{v}_2 \hat{n} \cdot \vec{a}_2 - \hat{n} \times \vec{a}_2 \cdot \vec{S}_1 \hat{n} \cdot \vec{v}_1 - \frac{27}{25} \hat{n} \times \vec{S}_1 \cdot \vec{v}_2 \hat{n} \cdot \vec{v}_2 - \right.$$

$$\left. \frac{1}{25} \hat{n} \times \vec{a}_2 \cdot \vec{S}_1 \hat{n} \cdot \vec{v}_2 - \vec{a}_2 \times \vec{S}_1 \cdot \vec{v}_2 \log\left(\frac{r}{R_\theta}\right) + \frac{6}{5} \hat{n} \times \vec{S}_1 \cdot \vec{v}_2 \hat{n} \cdot \vec{a}_2 \log\left(\frac{r}{R_\theta}\right) + \frac{3}{5} \hat{n} \times \vec{S}_1 \cdot \vec{v}_2 \hat{n} \cdot \vec{v}_2 \log\left(\frac{r}{R_\theta}\right) + \right.$$

$$\left. \frac{9}{5} \hat{n} \times \vec{a}_2 \cdot \vec{S}_1 \hat{n} \cdot \vec{v}_2 \log\left(\frac{r}{R_\theta}\right) + \frac{\frac{1}{3} \vec{a}_2 \times \vec{S}_1 \cdot \vec{v}_2 - \frac{2}{5} \hat{n} \times \vec{S}_1 \cdot \vec{v}_2 \hat{n} \cdot \vec{a}_2 - \frac{1}{5} \hat{n} \times \vec{S}_1 \cdot \vec{v}_2 \hat{n} \cdot \vec{v}_2 - \frac{3}{5} \hat{n} \times \vec{a}_2 \cdot \vec{S}_1 \hat{n} \cdot \vec{v}_2}{\epsilon_d} \right) m_2^3 + \frac{1}{r^4}$$

$$G^3 \left( \frac{15}{49} \hat{n} \times \vec{S}_1 \cdot \vec{v}_2 (\hat{n} \cdot \vec{v}_2)^2 - \frac{6}{7} \hat{n} \times \vec{S}_1 \cdot \vec{v}_2 \log\left(\frac{r}{R_\theta}\right) (\hat{n} \cdot \vec{v}_2)^2 + \frac{27}{25} \vec{S}_1 \times \vec{v}_1 \cdot \vec{v}_2 \hat{n} \cdot \vec{v}_2 + 6 \hat{n} \times \vec{S}_1 \cdot \vec{v}_2 \hat{n} \cdot \vec{v}_1 \hat{n} \cdot \vec{v}_2 - \right.$$

$$\left. \frac{3}{5} \vec{S}_1 \times \vec{v}_1 \cdot \vec{v}_2 \log\left(\frac{r}{R_\theta}\right) \hat{n} \cdot \vec{v}_2 - 3 \hat{n} \times \vec{S}_1 \cdot \vec{v}_2 \hat{n} \cdot \vec{v}_1 \log\left(\frac{r}{R_\theta}\right) \hat{n} \cdot \vec{v}_2 - \frac{27}{25} \hat{n} \times \vec{S}_1 \cdot \vec{v}_2 \vec{v}_1 \cdot \vec{v}_2 - \frac{453 \hat{n} \times \vec{S}_1 \cdot \vec{v}_2 \vec{v}_2 \cdot \vec{v}_2}{1225} + \right.$$

$$\left. \frac{3}{5} \hat{n} \times \vec{S}_1 \cdot \vec{v}_2 \vec{v}_1 \cdot \vec{v}_2 \log\left(\frac{r}{R_\theta}\right) + \frac{6}{35} \hat{n} \times \vec{S}_1 \cdot \vec{v}_2 \vec{v}_2 \cdot \vec{v}_2 \log\left(\frac{r}{R_\theta}\right) + \frac{1}{\epsilon_d} \left( \frac{2}{7} \hat{n} \times \vec{S}_1 \cdot \vec{v}_2 (\hat{n} \cdot \vec{v}_2)^2 + \right.$$

$$\left. \frac{1}{5} \vec{S}_1 \times \vec{v}_1 \cdot \vec{v}_2 \hat{n} \cdot \vec{v}_2 + \hat{n} \times \vec{S}_1 \cdot \vec{v}_2 \hat{n} \cdot \vec{v}_1 \hat{n} \cdot \vec{v}_2 - \frac{1}{5} \hat{n} \times \vec{S}_1 \cdot \vec{v}_2 \vec{v}_1 \cdot \vec{v}_2 - \frac{2}{35} \hat{n} \times \vec{S}_1 \cdot \vec{v}_2 \vec{v}_2 \cdot \vec{v}_2 \right) m_2^3 \}$$

{DiagSet[3, 1, 212],

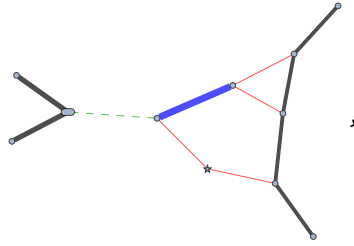

$$\frac{1}{r^3} G^3 m_2^3 \left( \frac{\frac{1}{10} \hat{n} \cdot \vec{v}_2 \hat{n} \times \vec{a}_2 \cdot \vec{S}_1 - \frac{1}{10} \hat{n} \cdot \vec{a}_2 \hat{n} \times \vec{S}_1 \cdot \vec{v}_2}{\epsilon_d} + \frac{3}{10} \log\left(\frac{r}{R_\theta}\right) \hat{n} \cdot \vec{a}_2 \hat{n} \times \vec{S}_1 \cdot \vec{v}_2 - \frac{3}{10} \log\left(\frac{r}{R_\theta}\right) \hat{n} \cdot \vec{v}_2 \hat{n} \times \vec{a}_2 \cdot \vec{S}_1 - \right.$$

$$\hat{n} \cdot \vec{a}_1 \hat{n} \times \vec{S}_1 \cdot \vec{v}_2 - \frac{27}{50} \hat{n} \cdot \vec{a}_2 \hat{n} \times \vec{S}_1 \cdot \vec{v}_2 + \hat{n} \cdot \vec{v}_1 \hat{n} \times \vec{a}_2 \cdot \vec{S}_1 - \frac{23}{50} \hat{n} \cdot \vec{v}_2 \hat{n} \times \vec{a}_2 \cdot \vec{S}_1 + \frac{1}{3} \vec{a}_1 \times \vec{S}_1 \cdot \vec{v}_2 - \frac{1}{3} \vec{a}_2 \times \vec{S}_1 \cdot \vec{v}_1 +$$

$$\left. \frac{1}{3} \vec{a}_2 \times \vec{S}_1 \cdot \vec{v}_2 - 2 \hat{n} \cdot \vec{v}_1 \hat{n} \times \vec{S}_1 \cdot \vec{v}_2 + \hat{n} \cdot \vec{v}_2 \hat{n} \times \vec{S}_1 \cdot \vec{v}_2 - \frac{2}{3} \vec{S}_1 \times \vec{v}_1 \cdot \vec{v}_2 \right) + \frac{G^3 m_2^3 \left( \frac{1}{3} \hat{n} \times \vec{S}_1 \cdot \vec{v}_2 - \frac{1}{3} \hat{n} \times \vec{a}_2 \cdot \vec{S}_1 \right)}{r^2} +$$

$$\frac{1}{r^4} G^3 m_2^3 \left( \frac{\frac{2}{35} \vec{v}_2 \cdot \vec{v}_2 \hat{n} \times \vec{S}_1 \cdot \vec{v}_2 - \frac{2}{7} (\hat{n} \cdot \vec{v}_2)^2 \hat{n} \times \vec{S}_1 \cdot \vec{v}_2}{\epsilon_d} + \frac{6}{7} \log\left(\frac{r}{R_\theta}\right) (\hat{n} \cdot \vec{v}_2)^2 \hat{n} \times \vec{S}_1 \cdot \vec{v}_2 - \right.$$

$$\frac{6}{35} \log\left(\frac{r}{R_\theta}\right) \vec{v}_2 \cdot \vec{v}_2 \hat{n} \times \vec{S}_1 \cdot \vec{v}_2 + 5 (\hat{n} \cdot \vec{v}_1)^2 \hat{n} \times \vec{S}_1 \cdot \vec{v}_2 + 2 \hat{n} \cdot \vec{v}_1 \vec{S}_1 \times \vec{v}_1 \cdot \vec{v}_2 - 5 \hat{n} \cdot \vec{v}_2 \hat{n} \cdot \vec{v}_1 \hat{n} \times \vec{S}_1 \cdot \vec{v}_2 -$$

$$\left. \frac{15}{49} (\hat{n} \cdot \vec{v}_2)^2 \hat{n} \times \vec{S}_1 \cdot \vec{v}_2 - \hat{n} \cdot \vec{v}_2 \vec{S}_1 \times \vec{v}_1 \cdot \vec{v}_2 - \vec{v}_1 \cdot \vec{v}_1 \hat{n} \times \vec{S}_1 \cdot \vec{v}_2 + \vec{v}_1 \cdot \vec{v}_2 \hat{n} \times \vec{S}_1 \cdot \vec{v}_2 + \frac{453 \vec{v}_2 \cdot \vec{v}_2 \hat{n} \times \vec{S}_1 \cdot \vec{v}_2}{1225} \right\}$$

{DiagSet[3, 1, 213],

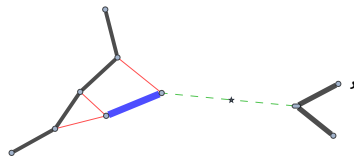

$$\frac{1}{r^3} G^3 m_2^3 \left( \frac{-\frac{1}{5} \hat{n} \cdot \vec{v}_1 \hat{n} \times \vec{a}_2 \cdot \vec{S}_1 + \frac{1}{15} \vec{a}_2 \times \vec{S}_1 \cdot \vec{v}_1 - \frac{1}{5} \hat{n} \cdot \vec{v}_2 \hat{n} \times \vec{S}_1 \cdot \vec{v}_2}{\epsilon_d} + \frac{3}{5} \log\left(\frac{r}{R_\theta}\right) \hat{n} \cdot \vec{v}_1 \hat{n} \times \vec{a}_2 \cdot \vec{S}_1 - \frac{17}{25} \hat{n} \cdot \vec{v}_1 \hat{n} \times \vec{a}_2 \cdot \vec{S}_1 - \right.$$

$$\left. \frac{1}{5} \log\left(\frac{r}{R_\theta}\right) \vec{a}_2 \times \vec{S}_1 \cdot \vec{v}_1 + \frac{4}{25} \vec{a}_2 \times \vec{S}_1 \cdot \vec{v}_1 + \frac{3}{5} \log\left(\frac{r}{R_\theta}\right) \hat{n} \cdot \vec{v}_2 \hat{n} \times \vec{S}_1 \cdot \vec{v}_2 - \frac{17}{25} \hat{n} \cdot \vec{v}_2 \hat{n} \times \vec{S}_1 \cdot \vec{v}_2 \right) +$$

$$\frac{G^3 m_2^3 \left( \frac{\hat{n} \times \vec{a}_2 \cdot \vec{S}_1}{15 \epsilon_d} - \frac{1}{5} \log\left(\frac{r}{R_\theta}\right) \hat{n} \times \vec{a}_2 \cdot \vec{S}_1 + \frac{4}{25} \hat{n} \times \vec{a}_2 \cdot \vec{S}_1 \right)}{r^2} + \frac{1}{r^4}$$

$$G^3 m_2^3 \left( \frac{\frac{1}{5} \hat{n} \cdot \vec{v}_2 \vec{S}_1 \times \vec{v}_1 \cdot \vec{v}_2 + \hat{n} \cdot \vec{v}_1 \hat{n} \cdot \vec{v}_2 \hat{n} \times \vec{S}_1 \cdot \vec{v}_2 - \frac{1}{5} \vec{v}_1 \cdot \vec{v}_2 \hat{n} \times \vec{S}_1 \cdot \vec{v}_2}{\epsilon_d} - \right.$$

$$\frac{3}{5} \log\left(\frac{r}{R_\theta}\right) \hat{n} \cdot \vec{v}_2 \vec{S}_1 \times \vec{v}_1 \cdot \vec{v}_2 - 3 \log\left(\frac{r}{R_\theta}\right) \hat{n} \cdot \vec{v}_1 \hat{n} \cdot \vec{v}_2 \hat{n} \times \vec{S}_1 \cdot \vec{v}_2 + \frac{3}{5} \log\left(\frac{r}{R_\theta}\right) \vec{v}_1 \cdot \vec{v}_2 \hat{n} \times \vec{S}_1 \cdot \vec{v}_2 +$$

$$\left. \frac{17}{25} \hat{n} \cdot \vec{v}_2 \vec{S}_1 \times \vec{v}_1 \cdot \vec{v}_2 + 4 \hat{n} \cdot \vec{v}_1 \hat{n} \cdot \vec{v}_2 \hat{n} \times \vec{S}_1 \cdot \vec{v}_2 - \frac{17}{25} \vec{v}_1 \cdot \vec{v}_2 \hat{n} \times \vec{S}_1 \cdot \vec{v}_2 \right\}$$

{DiagSet[3, 1, 214], 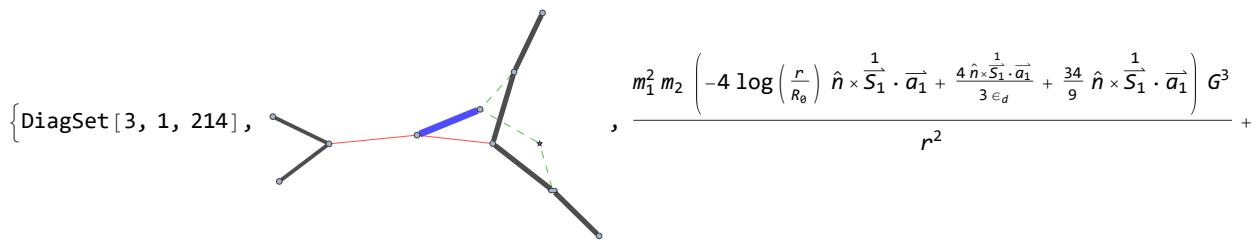

, 
$$\frac{m_1^2 m_2 \left( -4 \log\left(\frac{r}{R_\theta}\right) \hat{n} \times \vec{S}_1 \cdot \vec{a}_1 + \frac{4 \hat{n} \times \vec{S}_1 \cdot \vec{a}_1}{3 \in_d} + \frac{34}{9} \hat{n} \times \vec{S}_1 \cdot \vec{a}_1 \right) G^3}{r^2} +$$

$$\begin{aligned} & \frac{1}{r^3} m_1^2 m_2 \left( 4 \log\left(\frac{r}{R_\theta}\right) \vec{S}_1 \times \vec{v}_1 \cdot \vec{v}_2 - \frac{34}{9} \vec{S}_1 \times \vec{v}_1 \cdot \vec{v}_2 + \frac{4}{75} \vec{S}_1 \times \vec{v}_1 \cdot \vec{a}_1 - \frac{44}{25} \hat{n} \times \vec{S}_1 \cdot \vec{v}_1 \hat{n} \cdot \vec{a}_1 - \right. \\ & \frac{883}{75} \hat{n} \times \vec{S}_1 \cdot \vec{v}_1 \hat{n} \cdot \vec{v}_1 - \frac{9}{5} \hat{n} \times \vec{S}_1 \cdot \vec{a}_1 \hat{n} \cdot \vec{v}_1 + \frac{46}{3} \hat{n} \times \vec{S}_1 \cdot \vec{v}_1 \hat{n} \cdot \vec{v}_2 - \frac{7}{5} \vec{S}_1 \times \vec{v}_1 \cdot \vec{a}_1 \log\left(\frac{r}{R_\theta}\right) + \\ & \frac{21}{5} \hat{n} \times \vec{S}_1 \cdot \vec{v}_1 \hat{n} \cdot \vec{a}_1 \log\left(\frac{r}{R_\theta}\right) + \frac{39}{5} \hat{n} \times \vec{S}_1 \cdot \vec{v}_1 \hat{n} \cdot \vec{v}_1 \log\left(\frac{r}{R_\theta}\right) - 12 \hat{n} \times \vec{S}_1 \cdot \vec{v}_1 \hat{n} \cdot \vec{v}_2 \log\left(\frac{r}{R_\theta}\right) + \frac{1}{\epsilon_d} \\ & \left. \left( -\frac{4}{3} \vec{S}_1 \times \vec{v}_1 \cdot \vec{v}_2 + \frac{7}{15} \vec{S}_1 \times \vec{v}_1 \cdot \vec{a}_1 - \frac{7}{5} \hat{n} \times \vec{S}_1 \cdot \vec{v}_1 \hat{n} \cdot \vec{a}_1 - \frac{13}{5} \hat{n} \times \vec{S}_1 \cdot \vec{v}_1 \hat{n} \cdot \vec{v}_1 + 4 \hat{n} \times \vec{S}_1 \cdot \vec{v}_1 \hat{n} \cdot \vec{v}_2 \right) \right) G^3 + \\ & \frac{1}{r^4} m_1^2 m_2 \left( \frac{2222}{147} \hat{n} \times \vec{S}_1 \cdot \vec{v}_1 (\hat{n} \cdot \vec{v}_1)^2 - \frac{111}{7} \hat{n} \times \vec{S}_1 \cdot \vec{v}_1 \log\left(\frac{r}{R_\theta}\right) (\hat{n} \cdot \vec{v}_1)^2 + \frac{89}{25} \vec{S}_1 \times \vec{v}_1 \cdot \vec{v}_2 \hat{n} \cdot \vec{v}_1 - \right. \\ & 22 \hat{n} \times \vec{S}_1 \cdot \vec{v}_1 \hat{n} \cdot \vec{v}_2 \hat{n} \cdot \vec{v}_1 - \frac{21}{5} \vec{S}_1 \times \vec{v}_1 \cdot \vec{v}_2 \log\left(\frac{r}{R_\theta}\right) \hat{n} \cdot \vec{v}_1 + 21 \hat{n} \times \vec{S}_1 \cdot \vec{v}_1 \hat{n} \cdot \vec{v}_2 \log\left(\frac{r}{R_\theta}\right) \hat{n} \cdot \vec{v}_1 - \\ & \frac{11509 \hat{n} \times \vec{S}_1 \cdot \vec{v}_1 \vec{v}_1 \cdot \vec{v}_1}{3675} + \frac{89}{25} \hat{n} \times \vec{S}_1 \cdot \vec{v}_1 \vec{v}_1 \cdot \vec{v}_2 + \frac{111}{35} \hat{n} \times \vec{S}_1 \cdot \vec{v}_1 \vec{v}_1 \cdot \vec{v}_1 \log\left(\frac{r}{R_\theta}\right) - \\ & \frac{21}{5} \hat{n} \times \vec{S}_1 \cdot \vec{v}_1 \vec{v}_1 \cdot \vec{v}_2 \log\left(\frac{r}{R_\theta}\right) + \frac{1}{\epsilon_d} \left( \frac{37}{7} \hat{n} \times \vec{S}_1 \cdot \vec{v}_1 (\hat{n} \cdot \vec{v}_1)^2 + \frac{7}{5} \vec{S}_1 \times \vec{v}_1 \cdot \vec{v}_2 \hat{n} \cdot \vec{v}_1 - \right. \\ & \left. \left. 7 \hat{n} \times \vec{S}_1 \cdot \vec{v}_1 \hat{n} \cdot \vec{v}_2 \hat{n} \cdot \vec{v}_1 - \frac{37}{35} \hat{n} \times \vec{S}_1 \cdot \vec{v}_1 \vec{v}_1 \cdot \vec{v}_1 + \frac{7}{5} \hat{n} \times \vec{S}_1 \cdot \vec{v}_1 \vec{v}_1 \cdot \vec{v}_2 \right) \right) G^3 \} \end{aligned}$$

{DiagSet[3, 1, 215], 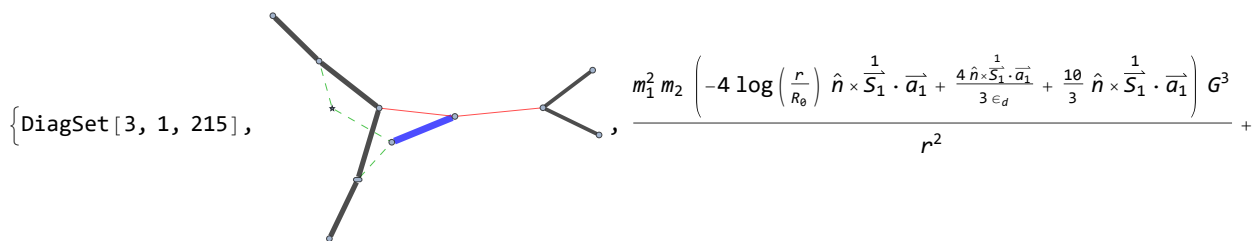

, 
$$\frac{m_1^2 m_2 \left( -4 \log\left(\frac{r}{R_\theta}\right) \hat{n} \times \vec{S}_1 \cdot \vec{a}_1 + \frac{4 \hat{n} \times \vec{S}_1 \cdot \vec{a}_1}{3 \in_d} + \frac{10}{3} \hat{n} \times \vec{S}_1 \cdot \vec{a}_1 \right) G^3}{r^2} +$$

$$\begin{aligned} & \frac{1}{r^3} m_1^2 m_2 \left( 4 \log\left(\frac{r}{R_\theta}\right) \vec{S}_1 \times \vec{a}_1 \cdot \vec{v}_2 - \frac{10}{3} \vec{S}_1 \times \vec{a}_1 \cdot \vec{v}_2 - \frac{254}{75} \vec{S}_1 \times \vec{v}_1 \cdot \vec{a}_1 - \frac{39}{25} \hat{n} \times \vec{S}_1 \cdot \vec{v}_1 \hat{n} \cdot \vec{a}_1 + \frac{52}{25} \hat{n} \times \vec{S}_1 \cdot \vec{v}_1 \hat{n} \cdot \vec{v}_1 - \right. \\ & \frac{363}{25} \hat{n} \times \vec{S}_1 \cdot \vec{a}_1 \hat{n} \cdot \vec{v}_1 + 14 \hat{n} \times \vec{S}_1 \cdot \vec{a}_1 \hat{n} \cdot \vec{v}_2 + \frac{22}{5} \vec{S}_1 \times \vec{v}_1 \cdot \vec{a}_1 \log\left(\frac{r}{R_\theta}\right) + \frac{6}{5} \hat{n} \times \vec{S}_1 \cdot \vec{v}_1 \hat{n} \cdot \vec{a}_1 \log\left(\frac{r}{R_\theta}\right) - \\ & \frac{18}{5} \hat{n} \times \vec{S}_1 \cdot \vec{v}_1 \hat{n} \cdot \vec{v}_1 \log\left(\frac{r}{R_\theta}\right) + \frac{72}{5} \hat{n} \times \vec{S}_1 \cdot \vec{a}_1 \hat{n} \cdot \vec{v}_1 \log\left(\frac{r}{R_\theta}\right) - 12 \hat{n} \times \vec{S}_1 \cdot \vec{a}_1 \hat{n} \cdot \vec{v}_2 \log\left(\frac{r}{R_\theta}\right) + \frac{1}{\epsilon_d} \left( -\frac{4}{3} \vec{S}_1 \times \vec{a}_1 \cdot \vec{v}_2 - \right. \\ & \left. \frac{22}{15} \vec{S}_1 \times \vec{v}_1 \cdot \vec{a}_1 - \frac{2}{5} \hat{n} \times \vec{S}_1 \cdot \vec{v}_1 \hat{n} \cdot \vec{a}_1 + \frac{6}{5} \hat{n} \times \vec{S}_1 \cdot \vec{v}_1 \hat{n} \cdot \vec{v}_1 - \frac{24}{5} \hat{n} \times \vec{S}_1 \cdot \vec{a}_1 \hat{n} \cdot \vec{v}_1 + 4 \hat{n} \times \vec{S}_1 \cdot \vec{a}_1 \hat{n} \cdot \vec{v}_2 \right) \right) G^3 + \frac{1}{r^4} \\ & m_1^2 m_2 \left( -\frac{356}{49} \hat{n} \times \vec{S}_1 \cdot \vec{v}_1 (\hat{n} \cdot \vec{v}_1)^2 + \frac{78}{7} \hat{n} \times \vec{S}_1 \cdot \vec{v}_1 \log\left(\frac{r}{R_\theta}\right) (\hat{n} \cdot \vec{v}_1)^2 - \frac{52}{25} \vec{S}_1 \times \vec{v}_1 \cdot \vec{v}_2 \hat{n} \cdot \vec{v}_1 + 14 \hat{n} \times \vec{S}_1 \cdot \vec{v}_1 \hat{n} \cdot \vec{v}_2 \hat{n} \cdot \vec{v}_1 + \right. \\ & \frac{18}{5} \vec{S}_1 \times \vec{v}_1 \cdot \vec{v}_2 \log\left(\frac{r}{R_\theta}\right) \hat{n} \cdot \vec{v}_1 - 18 \hat{n} \times \vec{S}_1 \cdot \vec{v}_1 \hat{n} \cdot \vec{v}_2 \log\left(\frac{r}{R_\theta}\right) \hat{n} \cdot \vec{v}_1 - \frac{166 \hat{n} \times \vec{S}_1 \cdot \vec{v}_1 \vec{v}_1 \cdot \vec{v}_1}{1225} - \frac{52}{25} \hat{n} \times \vec{S}_1 \cdot \vec{v}_1 \vec{v}_1 \cdot \vec{v}_2 - \\ & \left. \frac{78}{35} \hat{n} \times \vec{S}_1 \cdot \vec{v}_1 \vec{v}_1 \cdot \vec{v}_1 \log\left(\frac{r}{R_\theta}\right) + \frac{18}{5} \hat{n} \times \vec{S}_1 \cdot \vec{v}_1 \vec{v}_1 \cdot \vec{v}_2 \log\left(\frac{r}{R_\theta}\right) + \frac{1}{\epsilon_d} \left( -\frac{26}{7} \hat{n} \times \vec{S}_1 \cdot \vec{v}_1 (\hat{n} \cdot \vec{v}_1)^2 - \right. \right. \end{aligned}$$

$$\left. \frac{6}{5} \vec{S}_1 \times \vec{v}_1 \cdot \vec{v}_2 \hat{n} \cdot \vec{v}_1 + 6 \hat{n} \times \vec{S}_1 \cdot \vec{v}_1 \hat{n} \cdot \vec{v}_2 \hat{n} \cdot \vec{v}_1 + \frac{26}{35} \hat{n} \times \vec{S}_1 \cdot \vec{v}_1 \vec{v}_1 \cdot \vec{v}_1 - \frac{6}{5} \hat{n} \times \vec{S}_1 \cdot \vec{v}_1 \vec{v}_1 \cdot \vec{v}_2 \right) G^3 \Bigg\}$$

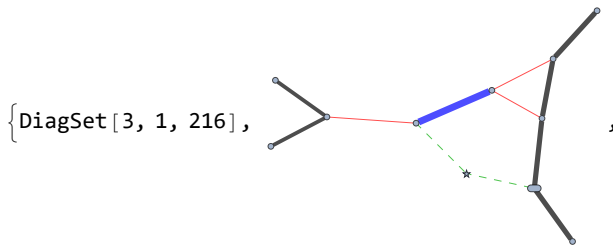

$$\begin{aligned} & \frac{m_1^2 m_2 \left( -\frac{1}{2} \log\left(\frac{r}{R_\theta}\right) \hat{n} \times \vec{S}_1 \cdot \vec{v}_1 + \frac{\hat{n} \times \vec{S}_1 \cdot \vec{v}_1}{6 \in_d} + \frac{1}{2} \hat{n} \times \vec{S}_1 \cdot \vec{v}_1 \right) G^3}{r^2} + \frac{1}{r^3} m_1^2 m_2 \left( -\frac{1}{2} \log\left(\frac{r}{R_\theta}\right) \vec{S}_1 \times \vec{v}_1 \cdot \vec{v}_2 + \frac{1}{2} \vec{S}_1 \times \vec{v}_1 \cdot \vec{v}_2 + \right. \\ & \frac{1}{2} \vec{S}_1 \times \vec{a}_1 \cdot \vec{v}_2 + \frac{1}{2} \vec{S}_1 \times \vec{v}_1 \cdot \vec{a}_1 + \frac{1}{2} \vec{S}_1 \times \vec{v}_1 \cdot \vec{a}_2 - \frac{39}{50} \hat{n} \times \vec{S}_1 \cdot \vec{v}_1 \hat{n} \cdot \vec{a}_1 - 2 \hat{n} \times \vec{S}_1 \cdot \vec{v}_1 \hat{n} \cdot \vec{a}_2 + \frac{22}{25} \hat{n} \times \vec{S}_1 \cdot \vec{v}_1 \hat{n} \cdot \vec{v}_1 + \\ & \frac{61}{50} \hat{n} \times \vec{S}_1 \cdot \vec{a}_1 \hat{n} \cdot \vec{v}_1 - 2 \hat{n} \times \vec{S}_1 \cdot \vec{v}_1 \hat{n} \cdot \vec{v}_2 - 2 \hat{n} \times \vec{S}_1 \cdot \vec{a}_1 \hat{n} \cdot \vec{v}_2 - \frac{1}{2} \vec{S}_1 \times \vec{a}_1 \cdot \vec{v}_2 \log\left(\frac{r}{R_\theta}\right) - \frac{1}{2} \vec{S}_1 \times \vec{v}_1 \cdot \vec{a}_1 \log\left(\frac{r}{R_\theta}\right) - \\ & \frac{1}{2} \vec{S}_1 \times \vec{v}_1 \cdot \vec{a}_2 \log\left(\frac{r}{R_\theta}\right) + \frac{3}{5} \hat{n} \times \vec{S}_1 \cdot \vec{v}_1 \hat{n} \cdot \vec{a}_1 \log\left(\frac{r}{R_\theta}\right) + \frac{3}{2} \hat{n} \times \vec{S}_1 \cdot \vec{v}_1 \hat{n} \cdot \vec{a}_2 \log\left(\frac{r}{R_\theta}\right) - \frac{3}{5} \hat{n} \times \vec{S}_1 \cdot \vec{v}_1 \hat{n} \cdot \vec{v}_1 \log\left(\frac{r}{R_\theta}\right) - \\ & \frac{9}{10} \hat{n} \times \vec{S}_1 \cdot \vec{a}_1 \hat{n} \cdot \vec{v}_1 \log\left(\frac{r}{R_\theta}\right) + \frac{3}{2} \hat{n} \times \vec{S}_1 \cdot \vec{v}_1 \hat{n} \cdot \vec{v}_2 \log\left(\frac{r}{R_\theta}\right) + \frac{3}{2} \hat{n} \times \vec{S}_1 \cdot \vec{a}_1 \hat{n} \cdot \vec{v}_2 \log\left(\frac{r}{R_\theta}\right) + \frac{1}{\in_d} \\ & \left. \left( \frac{1}{6} \vec{S}_1 \times \vec{v}_1 \cdot \vec{v}_2 + \frac{1}{6} \vec{S}_1 \times \vec{a}_1 \cdot \vec{v}_2 + \frac{1}{6} \vec{S}_1 \times \vec{v}_1 \cdot \vec{a}_1 + \frac{1}{6} \vec{S}_1 \times \vec{v}_1 \cdot \vec{a}_2 - \frac{1}{5} \hat{n} \times \vec{S}_1 \cdot \vec{v}_1 \hat{n} \cdot \vec{a}_1 - \frac{1}{2} \hat{n} \times \vec{S}_1 \cdot \vec{v}_1 \hat{n} \cdot \vec{a}_2 + \right. \right. \\ & \left. \left. \frac{1}{5} \hat{n} \times \vec{S}_1 \cdot \vec{v}_1 \hat{n} \cdot \vec{v}_1 + \frac{3}{10} \hat{n} \times \vec{S}_1 \cdot \vec{a}_1 \hat{n} \cdot \vec{v}_1 - \frac{1}{2} \hat{n} \times \vec{S}_1 \cdot \vec{v}_1 \hat{n} \cdot \vec{v}_2 - \frac{1}{2} \hat{n} \times \vec{S}_1 \cdot \vec{a}_1 \hat{n} \cdot \vec{v}_2 \right) \right) G^3 + \frac{1}{r^4} \\ & m_1^2 m_2 \left( -\frac{81}{98} \hat{n} \times \vec{S}_1 \cdot \vec{v}_1 (\hat{n} \cdot \vec{v}_1)^2 + \frac{3}{14} \hat{n} \times \vec{S}_1 \cdot \vec{v}_1 \log\left(\frac{r}{R_\theta}\right) (\hat{n} \cdot \vec{v}_1)^2 - 2 \vec{S}_1 \times \vec{v}_1 \cdot \vec{v}_2 \hat{n} \cdot \vec{v}_1 + \frac{23}{2} \hat{n} \times \vec{S}_1 \cdot \vec{v}_1 \hat{n} \cdot \vec{v}_2 \hat{n} \cdot \vec{v}_1 + \right. \\ & \frac{3}{2} \vec{S}_1 \times \vec{v}_1 \cdot \vec{v}_2 \log\left(\frac{r}{R_\theta}\right) \hat{n} \cdot \vec{v}_1 - \frac{15}{2} \hat{n} \times \vec{S}_1 \cdot \vec{v}_1 \hat{n} \cdot \vec{v}_2 \log\left(\frac{r}{R_\theta}\right) \hat{n} \cdot \vec{v}_1 - \frac{23}{2} \hat{n} \times \vec{S}_1 \cdot \vec{v}_1 (\hat{n} \cdot \vec{v}_2)^2 + 4 \vec{S}_1 \times \vec{v}_1 \cdot \vec{v}_2 \hat{n} \cdot \vec{v}_2 - \\ & \frac{438 \hat{n} \times \vec{S}_1 \cdot \vec{v}_1 \vec{v}_1 \cdot \vec{v}_1}{1225} - 2 \hat{n} \times \vec{S}_1 \cdot \vec{v}_1 \vec{v}_1 \cdot \vec{v}_2 + 2 \hat{n} \times \vec{S}_1 \cdot \vec{v}_1 \vec{v}_2 \cdot \vec{v}_2 + \frac{15}{2} \hat{n} \times \vec{S}_1 \cdot \vec{v}_1 (\hat{n} \cdot \vec{v}_2)^2 \log\left(\frac{r}{R_\theta}\right) - \\ & 3 \vec{S}_1 \times \vec{v}_1 \cdot \vec{v}_2 \hat{n} \cdot \vec{v}_2 \log\left(\frac{r}{R_\theta}\right) - \frac{3}{70} \hat{n} \times \vec{S}_1 \cdot \vec{v}_1 \vec{v}_1 \cdot \vec{v}_1 \log\left(\frac{r}{R_\theta}\right) + \frac{3}{2} \hat{n} \times \vec{S}_1 \cdot \vec{v}_1 \vec{v}_1 \cdot \vec{v}_2 \log\left(\frac{r}{R_\theta}\right) - \\ & \frac{3}{2} \hat{n} \times \vec{S}_1 \cdot \vec{v}_1 \vec{v}_2 \cdot \vec{v}_2 \log\left(\frac{r}{R_\theta}\right) + \frac{1}{\in_d} \left( -\frac{1}{14} \hat{n} \times \vec{S}_1 \cdot \vec{v}_1 (\hat{n} \cdot \vec{v}_1)^2 - \frac{1}{2} \vec{S}_1 \times \vec{v}_1 \cdot \vec{v}_2 \hat{n} \cdot \vec{v}_1 + \frac{5}{2} \hat{n} \times \vec{S}_1 \cdot \vec{v}_1 \hat{n} \cdot \vec{v}_2 \hat{n} \cdot \vec{v}_1 - \right. \\ & \left. \left. \frac{5}{2} \hat{n} \times \vec{S}_1 \cdot \vec{v}_1 (\hat{n} \cdot \vec{v}_2)^2 + \vec{S}_1 \times \vec{v}_1 \cdot \vec{v}_2 \hat{n} \cdot \vec{v}_2 + \frac{1}{70} \hat{n} \times \vec{S}_1 \cdot \vec{v}_1 \vec{v}_1 \cdot \vec{v}_1 - \frac{1}{2} \hat{n} \times \vec{S}_1 \cdot \vec{v}_1 \vec{v}_1 \cdot \vec{v}_2 + \frac{1}{2} \hat{n} \times \vec{S}_1 \cdot \vec{v}_1 \vec{v}_2 \cdot \vec{v}_2 \right) \right) G^3 \Bigg\} \end{aligned}$$

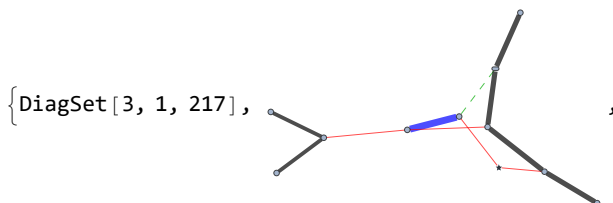

$$\frac{1}{r^2} m_1^2 m_2 \left( 3 \log\left(\frac{r}{R_\theta}\right) \hat{n} \times \vec{S}_1 \cdot \vec{a}_1 - \frac{5}{2} \hat{n} \times \vec{S}_1 \cdot \vec{a}_1 - \frac{11}{18} \hat{n} \times \vec{S}_1 \cdot \vec{v}_1 + \hat{n} \times \vec{S}_1 \cdot \vec{v}_1 \log\left(\frac{r}{R_\theta}\right) + \frac{-\left(\hat{n} \times \vec{S}_1 \cdot \vec{a}_1\right) - \frac{1}{3} \hat{n} \times \vec{S}_1 \cdot \vec{v}_1}{\in_d} \right) G^3 +$$



$$\begin{aligned} & \frac{1}{r^3} m_1^2 m_2 \left( -\log\left(\frac{r}{R_\theta}\right) \frac{1}{S_1} \times \vec{v}_1 \cdot \vec{v}_2 + \frac{11}{18} \frac{1}{S_1} \times \vec{v}_1 \cdot \vec{v}_2 + \frac{5}{2} \vec{S}_1 \times \vec{a}_1 \cdot \vec{v}_2 + \frac{74}{75} \vec{S}_1 \times \vec{v}_1 \cdot \vec{a}_1 + \frac{19}{6} \hat{n} \times \vec{S}_1 \cdot \vec{v}_1 \hat{n} \cdot \vec{a}_1 + \frac{673}{150} \hat{n} \times \vec{S}_1 \cdot \vec{v}_1 \hat{n} \cdot \vec{v}_1 + \right. \\ & \frac{632}{75} \hat{n} \times \vec{S}_1 \cdot \vec{a}_1 \hat{n} \cdot \vec{v}_1 - \frac{17}{6} \hat{n} \times \vec{S}_1 \cdot \vec{v}_1 \hat{n} \cdot \vec{v}_2 - \frac{21}{2} \hat{n} \times \vec{S}_1 \cdot \vec{a}_1 \hat{n} \cdot \vec{v}_2 - 3 \vec{S}_1 \times \vec{a}_1 \cdot \vec{v}_2 \log\left(\frac{r}{R_\theta}\right) - \frac{9}{10} \vec{S}_1 \times \vec{v}_1 \cdot \vec{a}_1 \log\left(\frac{r}{R_\theta}\right) - \\ & \frac{9}{2} \hat{n} \times \vec{S}_1 \cdot \vec{v}_1 \hat{n} \cdot \vec{a}_1 \log\left(\frac{r}{R_\theta}\right) - \frac{39}{10} \hat{n} \times \vec{S}_1 \cdot \vec{v}_1 \hat{n} \cdot \vec{v}_1 \log\left(\frac{r}{R_\theta}\right) - \frac{36}{5} \hat{n} \times \vec{S}_1 \cdot \vec{a}_1 \hat{n} \cdot \vec{v}_1 \log\left(\frac{r}{R_\theta}\right) + \\ & 3 \hat{n} \times \vec{S}_1 \cdot \vec{v}_1 \hat{n} \cdot \vec{v}_2 \log\left(\frac{r}{R_\theta}\right) + 9 \hat{n} \times \vec{S}_1 \cdot \vec{a}_1 \hat{n} \cdot \vec{v}_2 \log\left(\frac{r}{R_\theta}\right) + \frac{1}{\epsilon_d} \left( \frac{1}{3} \frac{1}{S_1} \times \vec{v}_1 \cdot \vec{v}_2 + \vec{S}_1 \times \vec{a}_1 \cdot \vec{v}_2 + \frac{3}{10} \vec{S}_1 \times \vec{v}_1 \cdot \vec{a}_1 + \right. \\ & \left. \frac{3}{2} \hat{n} \times \vec{S}_1 \cdot \vec{v}_1 \hat{n} \cdot \vec{a}_1 + \frac{13}{10} \hat{n} \times \vec{S}_1 \cdot \vec{v}_1 \hat{n} \cdot \vec{v}_1 + \frac{12}{5} \hat{n} \times \vec{S}_1 \cdot \vec{a}_1 \hat{n} \cdot \vec{v}_1 - \hat{n} \times \vec{S}_1 \cdot \vec{v}_1 \hat{n} \cdot \vec{v}_2 - 3 \hat{n} \times \vec{S}_1 \cdot \vec{a}_1 \hat{n} \cdot \vec{v}_2 \right) \Bigg) G^3 + \frac{1}{r^4} \\ & m_1^2 m_2 \left( -\frac{267}{49} \hat{n} \times \vec{S}_1 \cdot \vec{v}_1 (\hat{n} \cdot \vec{v}_1)^2 - \frac{9}{14} \hat{n} \times \vec{S}_1 \cdot \vec{v}_1 \log\left(\frac{r}{R_\theta}\right) (\hat{n} \cdot \vec{v}_1)^2 - \frac{22}{25} \vec{S}_1 \times \vec{v}_1 \cdot \vec{v}_2 \hat{n} \cdot \vec{v}_1 + \frac{7}{2} \hat{n} \times \vec{S}_1 \cdot \vec{v}_1 \hat{n} \cdot \vec{v}_2 \hat{n} \cdot \vec{v}_1 - \right. \\ & \frac{9}{10} \vec{S}_1 \times \vec{v}_1 \cdot \vec{v}_2 \log\left(\frac{r}{R_\theta}\right) \hat{n} \cdot \vec{v}_1 + \frac{9}{2} \hat{n} \times \vec{S}_1 \cdot \vec{v}_1 \hat{n} \cdot \vec{v}_2 \log\left(\frac{r}{R_\theta}\right) \hat{n} \cdot \vec{v}_1 + \frac{4553 \hat{n} \times \vec{S}_1 \cdot \vec{v}_1 \vec{v}_1 \cdot \vec{v}_1}{2450} - \frac{22}{25} \hat{n} \times \vec{S}_1 \cdot \vec{v}_1 \vec{v}_1 \cdot \vec{v}_2 + \\ & \frac{9}{70} \hat{n} \times \vec{S}_1 \cdot \vec{v}_1 \vec{v}_1 \cdot \vec{v}_1 \log\left(\frac{r}{R_\theta}\right) - \frac{9}{10} \hat{n} \times \vec{S}_1 \cdot \vec{v}_1 \vec{v}_1 \cdot \vec{v}_2 \log\left(\frac{r}{R_\theta}\right) + \frac{1}{\epsilon_d} \left( \frac{3}{14} \hat{n} \times \vec{S}_1 \cdot \vec{v}_1 (\hat{n} \cdot \vec{v}_1)^2 + \right. \\ & \left. \frac{3}{10} \vec{S}_1 \times \vec{v}_1 \cdot \vec{v}_2 \hat{n} \cdot \vec{v}_1 - \frac{3}{2} \hat{n} \times \vec{S}_1 \cdot \vec{v}_1 \hat{n} \cdot \vec{v}_2 \hat{n} \cdot \vec{v}_1 - \frac{3}{70} \hat{n} \times \vec{S}_1 \cdot \vec{v}_1 \vec{v}_1 \cdot \vec{v}_1 + \frac{3}{10} \hat{n} \times \vec{S}_1 \cdot \vec{v}_1 \vec{v}_1 \cdot \vec{v}_2 \right) \Bigg) G^3 \Bigg\} \end{aligned}$$

{DiagSet[3, 1, 218],

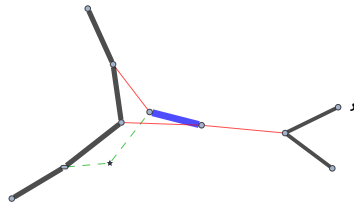

$$\begin{aligned} & \frac{1}{r^2} m_1^2 m_2 \left( \log\left(\frac{r}{R_\theta}\right) \hat{n} \times \vec{S}_1 \cdot \vec{a}_1 - \frac{19}{18} \hat{n} \times \vec{S}_1 \cdot \vec{a}_1 + \frac{13}{9} \hat{n} \times \vec{S}_1 \cdot \vec{v}_1 - 2 \hat{n} \times \vec{S}_1 \cdot \vec{v}_1 \log\left(\frac{r}{R_\theta}\right) + \frac{\frac{2}{3} \hat{n} \times \vec{S}_1 \cdot \vec{v}_1 - \frac{1}{3} \hat{n} \times \vec{S}_1 \cdot \vec{a}_1}{\epsilon_d} \right) G^3 + \\ & \frac{1}{r^3} m_1^2 m_2 \left( -5 \log\left(\frac{r}{R_\theta}\right) \frac{1}{S_1} \times \vec{v}_1 \cdot \vec{v}_2 + \frac{71}{18} \frac{1}{S_1} \times \vec{v}_1 \cdot \vec{v}_2 + \frac{13}{9} \vec{S}_1 \times \vec{a}_1 \cdot \vec{v}_2 + \frac{947}{450} \vec{S}_1 \times \vec{v}_1 \cdot \vec{a}_1 - \right. \\ & \frac{199}{150} \hat{n} \times \vec{S}_1 \cdot \vec{v}_1 \hat{n} \cdot \vec{a}_1 + \frac{2443}{150} \hat{n} \times \vec{S}_1 \cdot \vec{v}_1 \hat{n} \cdot \vec{v}_1 + \frac{1183}{150} \hat{n} \times \vec{S}_1 \cdot \vec{a}_1 \hat{n} \cdot \vec{v}_1 - \frac{101}{6} \hat{n} \times \vec{S}_1 \cdot \vec{v}_1 \hat{n} \cdot \vec{v}_2 - \\ & \frac{19}{3} \hat{n} \times \vec{S}_1 \cdot \vec{a}_1 \hat{n} \cdot \vec{v}_2 - 2 \vec{S}_1 \times \vec{a}_1 \cdot \vec{v}_2 \log\left(\frac{r}{R_\theta}\right) - \frac{27}{10} \vec{S}_1 \times \vec{v}_1 \cdot \vec{a}_1 \log\left(\frac{r}{R_\theta}\right) - \frac{3}{10} \hat{n} \times \vec{S}_1 \cdot \vec{v}_1 \hat{n} \cdot \vec{a}_1 \log\left(\frac{r}{R_\theta}\right) - \\ & \frac{159}{10} \hat{n} \times \vec{S}_1 \cdot \vec{v}_1 \hat{n} \cdot \vec{v}_1 \log\left(\frac{r}{R_\theta}\right) - \frac{42}{5} \hat{n} \times \vec{S}_1 \cdot \vec{a}_1 \hat{n} \cdot \vec{v}_1 \log\left(\frac{r}{R_\theta}\right) + 15 \hat{n} \times \vec{S}_1 \cdot \vec{v}_1 \hat{n} \cdot \vec{v}_2 \log\left(\frac{r}{R_\theta}\right) + \\ & 6 \hat{n} \times \vec{S}_1 \cdot \vec{a}_1 \hat{n} \cdot \vec{v}_2 \log\left(\frac{r}{R_\theta}\right) + \frac{1}{\epsilon_d} \left( \frac{5}{3} \frac{1}{S_1} \times \vec{v}_1 \cdot \vec{v}_2 + \frac{2}{3} \vec{S}_1 \times \vec{a}_1 \cdot \vec{v}_2 + \frac{9}{10} \vec{S}_1 \times \vec{v}_1 \cdot \vec{a}_1 + \frac{1}{10} \hat{n} \times \vec{S}_1 \cdot \vec{v}_1 \hat{n} \cdot \vec{a}_1 + \right. \\ & \left. \frac{53}{10} \hat{n} \times \vec{S}_1 \cdot \vec{v}_1 \hat{n} \cdot \vec{v}_1 + \frac{14}{5} \hat{n} \times \vec{S}_1 \cdot \vec{a}_1 \hat{n} \cdot \vec{v}_1 - 5 \hat{n} \times \vec{S}_1 \cdot \vec{v}_1 \hat{n} \cdot \vec{v}_2 - 2 \hat{n} \times \vec{S}_1 \cdot \vec{a}_1 \hat{n} \cdot \vec{v}_2 \right) \Bigg) G^3 + \frac{1}{r^4} \\ & m_1^2 m_2 \left( -\frac{174}{49} \hat{n} \times \vec{S}_1 \cdot \vec{v}_1 (\hat{n} \cdot \vec{v}_1)^2 + \frac{51}{14} \hat{n} \times \vec{S}_1 \cdot \vec{v}_1 \log\left(\frac{r}{R_\theta}\right) (\hat{n} \cdot \vec{v}_1)^2 - \frac{11}{25} \vec{S}_1 \times \vec{v}_1 \cdot \vec{v}_2 \hat{n} \cdot \vec{v}_1 + \frac{5}{2} \hat{n} \times \vec{S}_1 \cdot \vec{v}_1 \hat{n} \cdot \vec{v}_2 \hat{n} \cdot \vec{v}_1 + \right. \\ & \frac{3}{10} \vec{S}_1 \times \vec{v}_1 \cdot \vec{v}_2 \log\left(\frac{r}{R_\theta}\right) \hat{n} \cdot \vec{v}_1 - \frac{3}{2} \hat{n} \times \vec{S}_1 \cdot \vec{v}_1 \hat{n} \cdot \vec{v}_2 \log\left(\frac{r}{R_\theta}\right) \hat{n} \cdot \vec{v}_1 + \frac{2013 \hat{n} \times \vec{S}_1 \cdot \vec{v}_1 \vec{v}_1 \cdot \vec{v}_1}{2450} - \frac{11}{25} \hat{n} \times \vec{S}_1 \cdot \vec{v}_1 \vec{v}_1 \cdot \vec{v}_2 - \\ & \frac{51}{70} \hat{n} \times \vec{S}_1 \cdot \vec{v}_1 \vec{v}_1 \cdot \vec{v}_1 \log\left(\frac{r}{R_\theta}\right) + \frac{3}{10} \hat{n} \times \vec{S}_1 \cdot \vec{v}_1 \vec{v}_1 \cdot \vec{v}_2 \log\left(\frac{r}{R_\theta}\right) + \frac{1}{\epsilon_d} \left( -\frac{17}{14} \hat{n} \times \vec{S}_1 \cdot \vec{v}_1 (\hat{n} \cdot \vec{v}_1)^2 - \right. \end{aligned}$$

$$\frac{1}{10} \vec{S}_1 \times \vec{v}_1 \cdot \vec{v}_2 \hat{n} \cdot \vec{v}_1 + \frac{1}{2} \hat{n} \times \vec{S}_1 \cdot \vec{v}_1 \hat{n} \cdot \vec{v}_2 \hat{n} \cdot \vec{v}_1 + \frac{17}{70} \hat{n} \times \vec{S}_1 \cdot \vec{v}_1 \vec{v}_1 \cdot \vec{v}_1 - \frac{1}{10} \hat{n} \times \vec{S}_1 \cdot \vec{v}_1 \vec{v}_1 \cdot \vec{v}_2 \Big) G^3 \Big\}$$

{DiagSet[3, 1, 219],

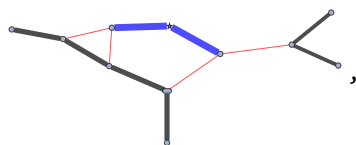

$$\frac{1}{r^3} G^3 m_1^2 m_2 \left( \frac{\frac{1}{5} \hat{n} \cdot \vec{v}_1 \hat{n} \times \vec{S}_1 \cdot \vec{a}_1 + \frac{1}{15} \vec{S}_1 \times \vec{v}_1 \cdot \vec{a}_1 + \frac{1}{5} \hat{n} \cdot \vec{v}_1 \hat{n} \times \vec{S}_1 \cdot \vec{v}_1}{\epsilon_d} - \frac{3}{5} \log\left(\frac{r}{R_0}\right) \hat{n} \cdot \vec{v}_1 \hat{n} \times \vec{S}_1 \cdot \vec{a}_1 + \frac{16}{75} \hat{n} \cdot \vec{v}_1 \hat{n} \times \vec{S}_1 \cdot \vec{a}_1 - \right.$$

$$\left. \frac{1}{5} \log\left(\frac{r}{R_0}\right) \vec{S}_1 \times \vec{v}_1 \cdot \vec{a}_1 + \frac{61}{225} \vec{S}_1 \times \vec{v}_1 \cdot \vec{a}_1 - \frac{3}{5} \log\left(\frac{r}{R_0}\right) \hat{n} \cdot \vec{v}_1 \hat{n} \times \vec{S}_1 \cdot \vec{v}_1 + \frac{16}{75} \hat{n} \cdot \vec{v}_1 \hat{n} \times \vec{S}_1 \cdot \vec{v}_1 \right) + \frac{1}{r^4} G^3 m_1^2 m_2 \left( \frac{1}{\epsilon_d} \right.$$

$$\left( -\frac{8}{7} (\hat{n} \cdot \vec{v}_1)^2 \hat{n} \times \vec{S}_1 \cdot \vec{v}_1 - \frac{1}{5} \hat{n} \cdot \vec{v}_1 \vec{S}_1 \times \vec{v}_1 \cdot \vec{v}_2 + \hat{n} \cdot \vec{v}_2 \hat{n} \cdot \vec{v}_1 \hat{n} \times \vec{S}_1 \cdot \vec{v}_1 + \frac{8}{35} \vec{v}_1 \cdot \vec{v}_1 \hat{n} \times \vec{S}_1 \cdot \vec{v}_1 - \frac{1}{5} \vec{v}_1 \cdot \vec{v}_2 \hat{n} \times \vec{S}_1 \cdot \vec{v}_1 \right) +$$

$$\frac{24}{7} \log\left(\frac{r}{R_0}\right) (\hat{n} \cdot \vec{v}_1)^2 \hat{n} \times \vec{S}_1 \cdot \vec{v}_1 + \frac{3}{5} \log\left(\frac{r}{R_0}\right) \hat{n} \cdot \vec{v}_1 \vec{S}_1 \times \vec{v}_1 \cdot \vec{v}_2 - 3 \log\left(\frac{r}{R_0}\right) \hat{n} \cdot \vec{v}_2 \hat{n} \cdot \vec{v}_1 \hat{n} \times \vec{S}_1 \cdot \vec{v}_1 -$$

$$\frac{24}{35} \log\left(\frac{r}{R_0}\right) \vec{v}_1 \cdot \vec{v}_1 \hat{n} \times \vec{S}_1 \cdot \vec{v}_1 + \frac{3}{5} \log\left(\frac{r}{R_0}\right) \vec{v}_1 \cdot \vec{v}_2 \hat{n} \times \vec{S}_1 \cdot \vec{v}_1 - \frac{334}{147} (\hat{n} \cdot \vec{v}_1)^2 \hat{n} \times \vec{S}_1 \cdot \vec{v}_1 -$$

$$\left. \frac{16}{75} \hat{n} \cdot \vec{v}_1 \vec{S}_1 \times \vec{v}_1 \cdot \vec{v}_2 + \frac{5}{3} \hat{n} \cdot \vec{v}_2 \hat{n} \cdot \vec{v}_1 \hat{n} \times \vec{S}_1 \cdot \vec{v}_1 + \frac{3266 \vec{v}_1 \cdot \vec{v}_1 \hat{n} \times \vec{S}_1 \cdot \vec{v}_1}{3675} - \frac{16}{75} \vec{v}_1 \cdot \vec{v}_2 \hat{n} \times \vec{S}_1 \cdot \vec{v}_1 \right\}$$

{DiagSet[3, 2, 1],

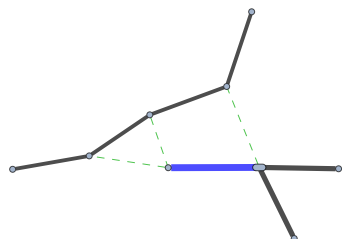

$$, -\frac{4 G^3 m_2^3 \vec{v}_2 \cdot \vec{v}_2 \hat{n} \times \vec{S}_1 \cdot \vec{v}_2}{r^4} \Big\}$$

{DiagSet[3, 2, 2],

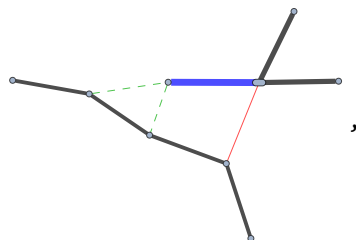

$$\frac{G^3 m_2^3 \left( -8 \hat{n} \cdot \vec{v}_2 \vec{S}_1 \times \vec{v}_1 \cdot \vec{v}_2 + 8 \vec{v}_1 \cdot \vec{v}_2 \hat{n} \times \vec{S}_1 \cdot \vec{v}_2 + 4 \vec{v}_2 \cdot \vec{v}_2 \hat{n} \times \vec{S}_1 \cdot \vec{v}_1 \right)}{r^4} \Big\}$$

{DiagSet[3, 2, 3],

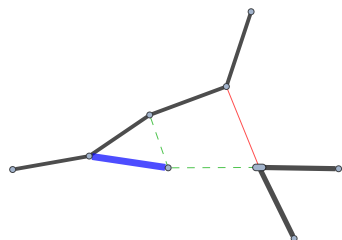

$$, \frac{G^3 m_2^3 \left( 32 \vec{v}_2 \cdot \vec{v}_2 \hat{n} \times \vec{S}_1 \cdot \vec{v}_2 - 128 (\hat{n} \cdot \vec{v}_2)^2 \hat{n} \times \vec{S}_1 \cdot \vec{v}_2 \right)}{r^4} \Big\}$$

{DiagSet[3, 2, 4],

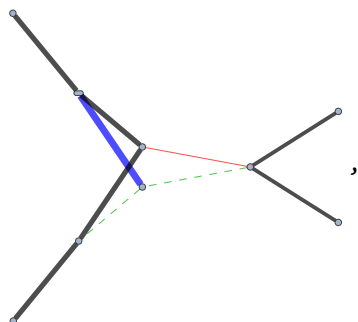

,

$$\frac{G^3 m_1^2 m_2 \left( 2 \hat{n} \cdot \vec{v}_1 \vec{S}_1 \times \vec{v}_1 \cdot \vec{v}_2 + 6 \vec{v}_1 \cdot \vec{v}_1 \hat{n} \times \vec{S}_1 \cdot \vec{v}_2 - 8 \vec{v}_1 \cdot \vec{v}_2 \hat{n} \times \vec{S}_1 \cdot \vec{v}_1 \right)}{r^4}$$

{DiagSet[3, 2, 5],

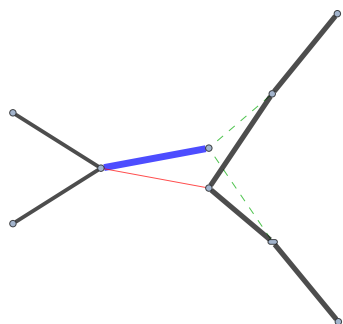

$$, \frac{G^3 m_1^2 m_2 \left( 6 \vec{v}_1 \cdot \vec{v}_2 \hat{n} \times \vec{S}_1 \cdot \vec{v}_2 - 12 (\hat{n} \cdot \vec{v}_2)^2 \hat{n} \times \vec{S}_1 \cdot \vec{v}_1 \right)}{r^4}$$

{DiagSet[3, 2, 6],

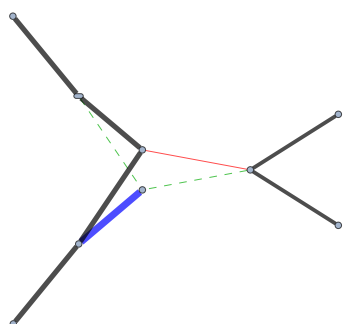

$$, \frac{1}{r^4}$$

$$G^3 m_1^2 m_2 \left( -24 (\hat{n} \cdot \vec{v}_1)^2 \hat{n} \times \vec{S}_1 \cdot \vec{v}_2 - 8 \hat{n} \cdot \vec{v}_1 \vec{S}_1 \times \vec{v}_1 \cdot \vec{v}_2 + 4 \vec{v}_1 \cdot \vec{v}_1 \hat{n} \times \vec{S}_1 \cdot \vec{v}_2 + 2 \vec{v}_1 \cdot \vec{v}_2 \hat{n} \times \vec{S}_1 \cdot \vec{v}_1 \right)$$

{DiagSet[3, 2, 7],

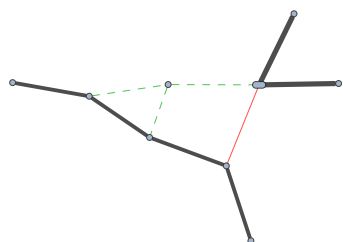

,

$$\frac{G^3 m_2^3 \left( 64 \hat{n} \cdot \vec{v}_2 \hat{n} \times \vec{S}_1 \cdot \vec{a}_2 + 32 \vec{S}_1 \times \vec{v}_2 \cdot \vec{a}_2 - 32 \hat{n} \cdot \vec{v}_2 \hat{n} \times \vec{S}_1 \cdot \vec{v}_2 \right)}{r^3} + \frac{1}{r^4} G^3 m_2^3$$

$$\left( 96 (\hat{n} \cdot \vec{v}_2)^2 \hat{n} \times \vec{S}_1 \cdot \vec{v}_2 + 32 \hat{n} \cdot \vec{v}_2 \vec{S}_1 \times \vec{v}_1 \cdot \vec{v}_2 + 160 \hat{n} \cdot \vec{v}_1 \hat{n} \cdot \vec{v}_2 \hat{n} \times \vec{S}_1 \cdot \vec{v}_2 - 32 \vec{v}_1 \cdot \vec{v}_2 \hat{n} \times \vec{S}_1 \cdot \vec{v}_2 - 24 \vec{v}_2 \cdot \vec{v}_2 \hat{n} \times \vec{S}_1 \cdot \vec{v}_2 \right)$$

{DiagSet[3, 2, 8],

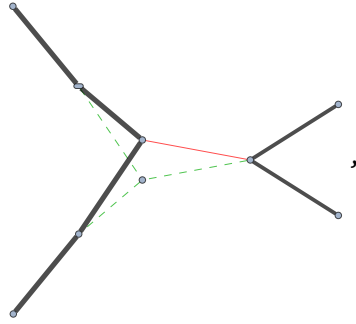

,

$$\frac{1}{r^3} G^3 m_1^2 m_2 \left( -6 \hat{n} \cdot \vec{v}_1 \hat{n} \times \vec{a}_2 \cdot \vec{S}_1 - 6 \hat{n} \cdot \vec{v}_2 \hat{n} \times \vec{a}_1 \cdot \vec{S}_1 + 2 \vec{a}_1 \times \vec{S}_1 \cdot \vec{v}_2 + \right. \\ \left. 2 \vec{a}_2 \times \vec{S}_1 \cdot \vec{v}_1 - 8 \hat{n} \cdot \vec{v}_1 \hat{n} \times \vec{S}_1 \cdot \vec{v}_2 + 2 \hat{n} \cdot \vec{v}_2 \hat{n} \times \vec{S}_1 \cdot \vec{v}_1 - 6 \vec{S}_1 \times \vec{v}_1 \cdot \vec{v}_2 \right) + \frac{1}{r^4} \\ G^3 m_1^2 m_2 \left( 18 (\hat{n} \cdot \vec{v}_1)^2 \hat{n} \times \vec{S}_1 \cdot \vec{v}_2 + 10 \hat{n} \cdot \vec{v}_1 \vec{S}_1 \times \vec{v}_1 \cdot \vec{v}_2 - 8 \hat{n} \cdot \vec{v}_2 \hat{n} \times \vec{S}_1 \cdot \vec{v}_1 + 30 \hat{n} \cdot \vec{v}_2 \hat{n} \times \vec{S}_1 \cdot \vec{v}_2 + \right. \\ \left. 6 \hat{n} \cdot \vec{v}_2 \vec{S}_1 \times \vec{v}_1 \cdot \vec{v}_2 - 6 \vec{v}_1 \cdot \vec{v}_1 \hat{n} \times \vec{S}_1 \cdot \vec{v}_2 + 6 \vec{v}_1 \cdot \vec{v}_2 \hat{n} \times \vec{S}_1 \cdot \vec{v}_1 - 6 \vec{v}_1 \cdot \vec{v}_2 \hat{n} \times \vec{S}_1 \cdot \vec{v}_2 \right) \Bigg\}$$

{DiagSet[3, 2, 9],

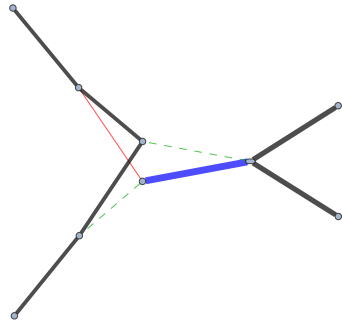

,

$$\frac{G^3 m_2^3 \left( -8 \hat{n} \cdot \vec{a}_2 \hat{n} \times \vec{S}_1 \cdot \vec{v}_2 - 8 \hat{n} \cdot \vec{v}_2 \hat{n} \times \vec{S}_1 \cdot \vec{a}_2 - 8 \vec{S}_1 \times \vec{v}_2 \cdot \vec{a}_2 \right)}{r^3} \Bigg\}$$

{DiagSet[3, 2, 10],

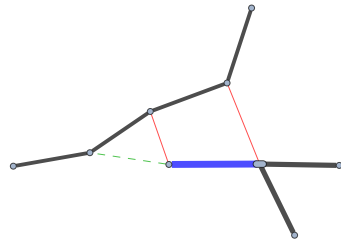

,

$$\frac{G^3 m_2^3 \left( 8 \hat{n} \cdot \vec{a}_2 \hat{n} \times \vec{S}_1 \cdot \vec{v}_1 - 8 \hat{n} \cdot \vec{v}_1 \hat{n} \times \vec{S}_1 \cdot \vec{a}_2 + 8 \vec{S}_1 \times \vec{v}_1 \cdot \vec{a}_2 \right)}{r^3} \Bigg\}$$

{DiagSet[3, 2, 11],

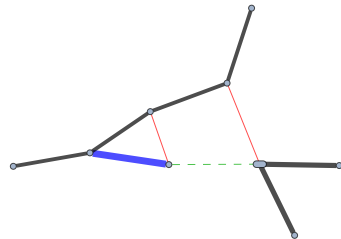

,

$$\frac{1}{r^4} G^3 m_2^3 \left( 160 (\hat{n} \cdot \vec{v}_2)^2 \hat{n} \times \vec{S}_1 \cdot \vec{v}_2 - 32 \hat{n} \cdot \vec{v}_2 \vec{S}_1 \times \vec{v}_1 \cdot \vec{v}_2 - 160 \hat{n} \cdot \vec{v}_1 \hat{n} \cdot \vec{v}_2 \hat{n} \times \vec{S}_1 \cdot \vec{v}_2 + \right. \\ \left. 32 \vec{v}_1 \cdot \vec{v}_2 \hat{n} \times \vec{S}_1 \cdot \vec{v}_2 - 32 \vec{v}_2 \cdot \vec{v}_2 \hat{n} \times \vec{S}_1 \cdot \vec{v}_2 \right) + \frac{32 G^3 m_2^3 \hat{n} \cdot \vec{v}_2 \hat{n} \times \vec{S}_1 \cdot \vec{v}_2}{r^3} \Bigg\}$$

$\left\{ \text{DiagSet}[3, 2, 12], \right.$ 
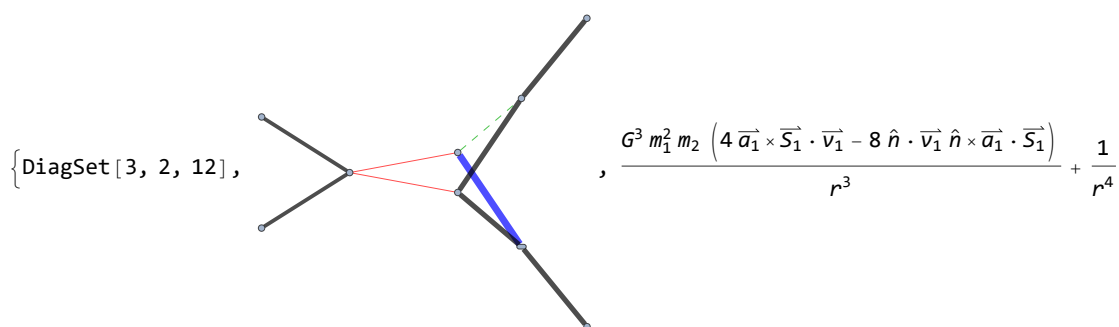
 $\left. , \frac{G^3 m_1^2 m_2 \left( 4 \vec{a}_1 \times \vec{S}_1 \cdot \vec{v}_1 - 8 \hat{n} \cdot \vec{v}_1 \hat{n} \times \vec{a}_1 \cdot \vec{S}_1 \right)}{r^3} + \frac{1}{r^4} \right\}$

$$G^3 m_1^2 m_2 \left( -10 \left( \hat{n} \cdot \vec{v}_1 \right)^2 \hat{n} \times \vec{S}_1 \cdot \vec{v}_1 - 2 \hat{n} \cdot \vec{v}_1 \vec{S}_1 \times \vec{v}_1 \cdot \vec{v}_2 + 10 \hat{n} \cdot \vec{v}_2 \hat{n} \cdot \vec{v}_1 \hat{n} \times \vec{S}_1 \cdot \vec{v}_1 - 2 \vec{v}_1 \cdot \vec{v}_2 \hat{n} \times \vec{S}_1 \cdot \vec{v}_1 \right) \Big\}$$

$\left\{ \text{DiagSet}[3, 2, 13], \right.$ 
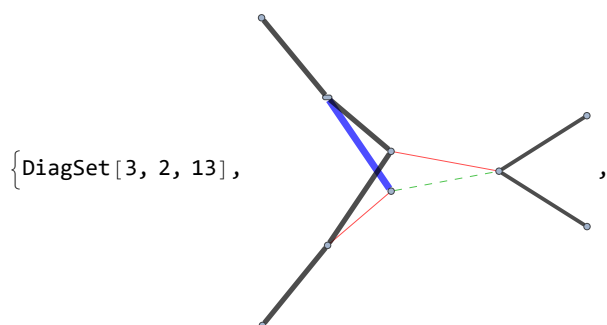
 $\left. , \right.$

$$\frac{G^3 m_1^2 m_2 \left( 2 \hat{n} \cdot \vec{v}_1 \hat{n} \times \vec{a}_2 \cdot \vec{S}_1 - 2 \vec{a}_2 \times \vec{S}_1 \cdot \vec{v}_1 \right)}{r^3} + \frac{1}{r^4} G^3 m_1^2 m_2 \left( 10 \left( \hat{n} \cdot \vec{v}_1 \right)^2 \hat{n} \times \vec{S}_1 \cdot \vec{v}_2 + 8 \hat{n} \cdot \vec{v}_1 \vec{S}_1 \times \vec{v}_1 \cdot \vec{v}_2 - \right. \\ \left. 10 \hat{n} \cdot \vec{v}_2 \hat{n} \cdot \vec{v}_1 \hat{n} \times \vec{S}_1 \cdot \vec{v}_2 - 6 \hat{n} \cdot \vec{v}_2 \vec{S}_1 \times \vec{v}_1 \cdot \vec{v}_2 - 2 \vec{v}_1 \cdot \vec{v}_1 \hat{n} \times \vec{S}_1 \cdot \vec{v}_2 + 2 \vec{v}_1 \cdot \vec{v}_2 \hat{n} \times \vec{S}_1 \cdot \vec{v}_1 + 2 \vec{v}_1 \cdot \vec{v}_2 \hat{n} \times \vec{S}_1 \cdot \vec{v}_2 \right) \Big\}$$

$\left\{ \text{DiagSet}[3, 2, 14], \right.$ 
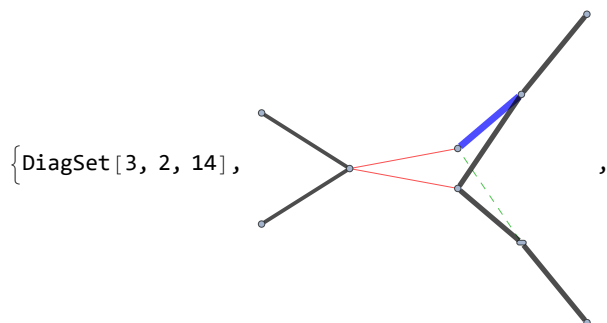
 $\left. , \right.$

$$\frac{1}{r^4} G^3 m_1^2 m_2 \left( -30 \left( \hat{n} \cdot \vec{v}_1 \right)^2 \hat{n} \times \vec{S}_1 \cdot \vec{v}_1 - 6 \hat{n} \cdot \vec{v}_1 \vec{S}_1 \times \vec{v}_1 \cdot \vec{v}_2 + 30 \hat{n} \cdot \vec{v}_2 \hat{n} \cdot \vec{v}_1 \hat{n} \times \vec{S}_1 \cdot \vec{v}_1 + \right. \\ \left. 6 \vec{v}_1 \cdot \vec{v}_1 \hat{n} \times \vec{S}_1 \cdot \vec{v}_1 - 6 \vec{v}_1 \cdot \vec{v}_2 \hat{n} \times \vec{S}_1 \cdot \vec{v}_1 \right) + \frac{8 G^3 m_1^2 m_2 \hat{n} \cdot \vec{v}_1 \hat{n} \times \vec{S}_1 \cdot \vec{v}_1}{r^3} \Big\}$$

$\left\{ \text{DiagSet}[3, 2, 15], \right.$ 
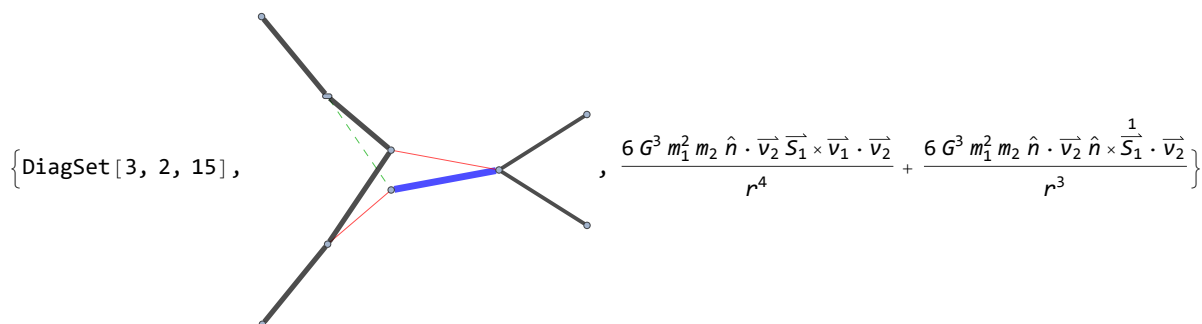
 $\left. , \frac{6 G^3 m_1^2 m_2 \hat{n} \cdot \vec{v}_2 \vec{S}_1 \times \vec{v}_1 \cdot \vec{v}_2}{r^4} + \frac{6 G^3 m_1^2 m_2 \hat{n} \cdot \vec{v}_2 \hat{n} \times \vec{S}_1 \cdot \vec{v}_2}{r^3} \right\}$

{DiagSet[3, 2, 16],

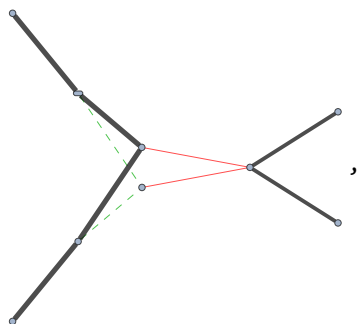

$$\frac{G^3 m_1^2 m_2 \left( 9 \vec{v}_2 \cdot \vec{v}_2 \hat{n} \times \vec{S}_1 \cdot \vec{v}_1 - 11 \vec{v}_1 \cdot \vec{v}_1 \hat{n} \times \vec{S}_1 \cdot \vec{v}_1 \right)}{r^4} - \frac{8 G^3 m_1^2 m_2 \vec{a}_1 \times \vec{S}_1 \cdot \vec{v}_1}{r^3} \}$$

{DiagSet[3, 2, 17],

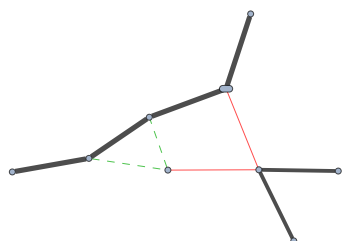

$$, - \frac{8 G^3 m_1^2 m_2 \vec{v}_1 \cdot \vec{v}_1 \hat{n} \times \vec{S}_1 \cdot \vec{v}_1}{r^4} \}$$

{DiagSet[3, 2, 18],

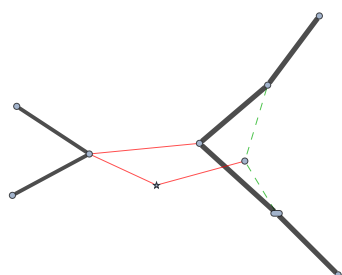

$$\frac{1}{r^3} G^3 m_1^2 m_2 \left( -\hat{n} \cdot \vec{v}_1 \hat{n} \times \vec{a}_1 \cdot \vec{S}_1 + 3 \hat{n} \cdot \vec{v}_2 \hat{n} \times \vec{a}_1 \cdot \vec{S}_1 - \vec{a}_1 \times \vec{S}_1 \cdot \vec{v}_2 + \hat{n} \cdot \vec{v}_1 \hat{n} \times \vec{S}_1 \cdot \vec{v}_1 - 3 \hat{n} \cdot \vec{v}_2 \hat{n} \times \vec{S}_1 \cdot \vec{v}_1 + \vec{S}_1 \times \vec{v}_1 \cdot \vec{v}_2 \right) +$$

$$\frac{1}{r^4} G^3 m_1^2 m_2 \left( -2 (\hat{n} \cdot \vec{v}_1)^2 \hat{n} \times \vec{S}_1 \cdot \vec{v}_1 - 2 \hat{n} \cdot \vec{v}_1 \vec{S}_1 \times \vec{v}_1 \cdot \vec{v}_2 + 10 \hat{n} \cdot \vec{v}_2 \hat{n} \cdot \vec{v}_1 \hat{n} \times \vec{S}_1 \cdot \vec{v}_1 - 2 \vec{v}_1 \cdot \vec{v}_2 \hat{n} \times \vec{S}_1 \cdot \vec{v}_1 \right) \}$$

{DiagSet[3, 2, 19],

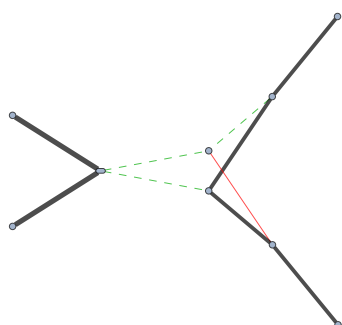

$$, \frac{32 G^3 m_2^3 \vec{S}_1 \times \vec{v}_2 \cdot \vec{a}_2}{r^3} - \frac{48 G^3 m_2^3 \vec{v}_1 \cdot \vec{v}_2 \hat{n} \times \vec{S}_1 \cdot \vec{v}_2}{r^4} \}$$

{DiagSet[3, 2, 20],

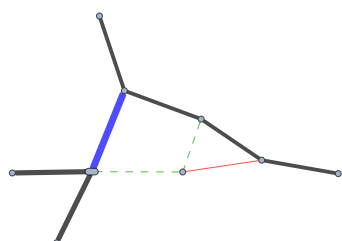

$$, - \frac{16 G^3 m_2^3 \vec{v}_2 \cdot \vec{v}_2 \hat{n} \times \vec{S}_1 \cdot \vec{v}_2}{r^4} \}$$

$\{\text{DiagSet}[3, 2, 21],$

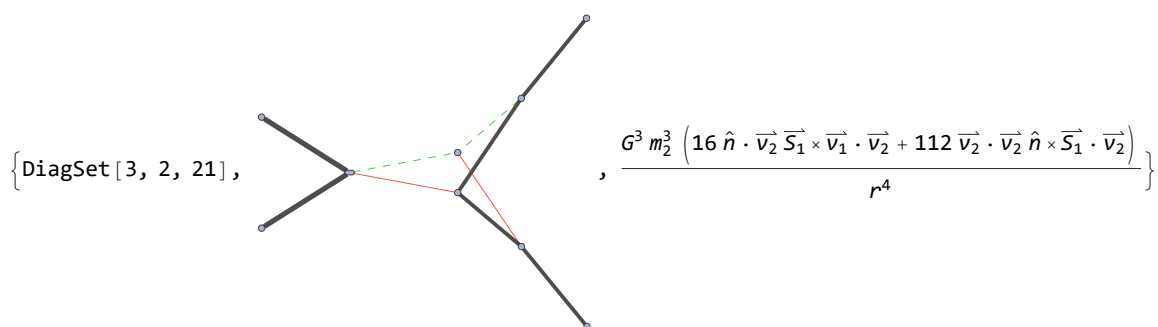

$, \frac{G^3 m_2^3 \left( 16 \hat{n} \cdot \vec{v}_2 \vec{S}_1 \times \vec{v}_1 \cdot \vec{v}_2 + 112 \vec{v}_2 \cdot \vec{v}_2 \hat{n} \times \vec{S}_1 \cdot \vec{v}_2 \right)}{r^4} \}$

$\{\text{DiagSet}[3, 2, 22],$

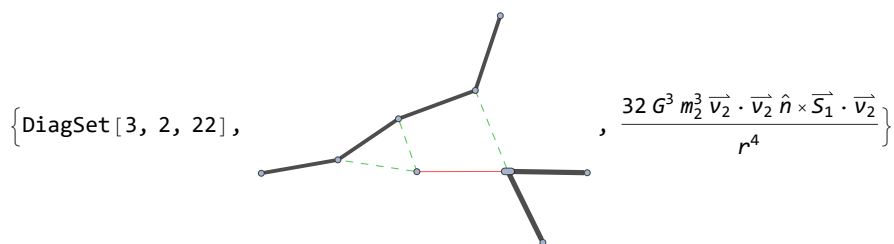

$, \frac{32 G^3 m_2^3 \vec{v}_2 \cdot \vec{v}_2 \hat{n} \times \vec{S}_1 \cdot \vec{v}_2}{r^4} \}$

$\{\text{DiagSet}[3, 2, 23],$

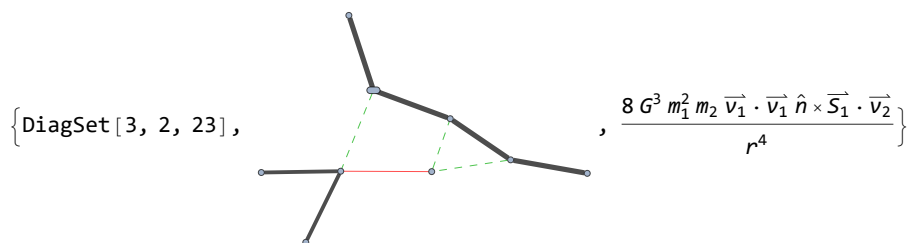

$, \frac{8 G^3 m_1^2 m_2 \vec{v}_1 \cdot \vec{v}_1 \hat{n} \times \vec{S}_1 \cdot \vec{v}_2}{r^4} \}$

$\{\text{DiagSet}[3, 2, 24],$

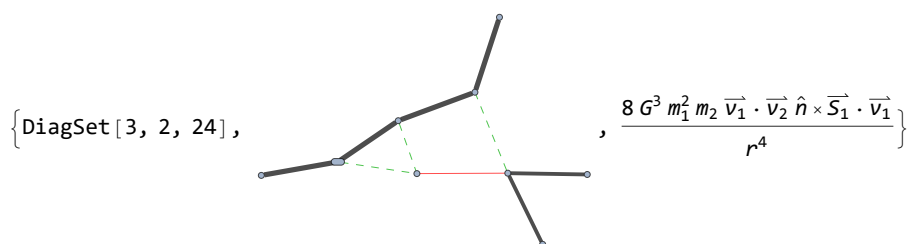

$, \frac{8 G^3 m_1^2 m_2 \vec{v}_1 \cdot \vec{v}_2 \hat{n} \times \vec{S}_1 \cdot \vec{v}_1}{r^4} \}$

$\{\text{DiagSet}[3, 2, 25],$

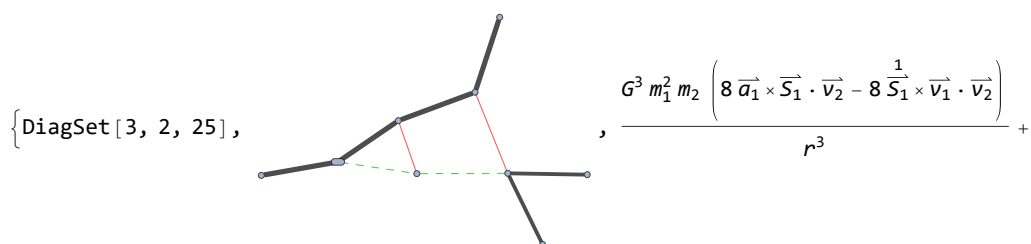

$, \frac{G^3 m_1^2 m_2 \left( 8 \vec{a}_1 \times \vec{S}_1 \cdot \vec{v}_2 - 8 \vec{S}_1 \times \vec{v}_1 \cdot \vec{v}_2 \right)}{r^3} +$

$\frac{1}{r^4} G^3 m_1^2 m_2 \left( 5 \hat{n} \cdot \vec{v}_1 \vec{S}_1 \times \vec{v}_1 \cdot \vec{v}_2 + 6 \vec{v}_1 \cdot \vec{v}_1 \hat{n} \times \vec{S}_1 \cdot \vec{v}_2 + 7 \vec{v}_1 \cdot \vec{v}_2 \hat{n} \times \vec{S}_1 \cdot \vec{v}_1 - 3 \vec{v}_2 \cdot \vec{v}_2 \hat{n} \times \vec{S}_1 \cdot \vec{v}_2 \right) \}$

$\{\text{DiagSet}[3, 2, 26],$

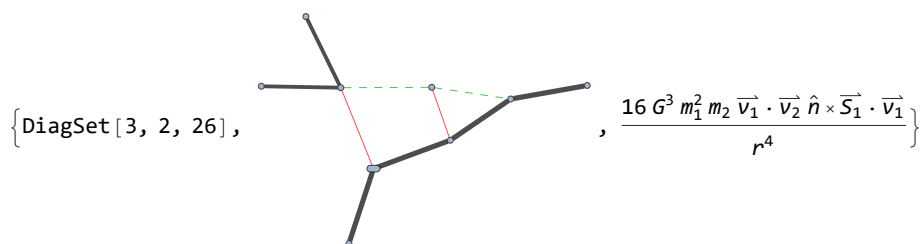

$, \frac{16 G^3 m_1^2 m_2 \vec{v}_1 \cdot \vec{v}_2 \hat{n} \times \vec{S}_1 \cdot \vec{v}_1}{r^4} \}$

$$\left\{ \text{DiagSet}[3, 2, 27], \right. , \left. \frac{G^3 m_1^2 m_2 \left( 16 \vec{v}_1 \cdot \vec{v}_2 \hat{n} \times \vec{S}_1 \cdot \vec{v}_1 - 8 \hat{n} \cdot \vec{v}_1 \vec{S}_1 \times \vec{v}_1 \cdot \vec{v}_2 \right)}{r^4} \right\}$$
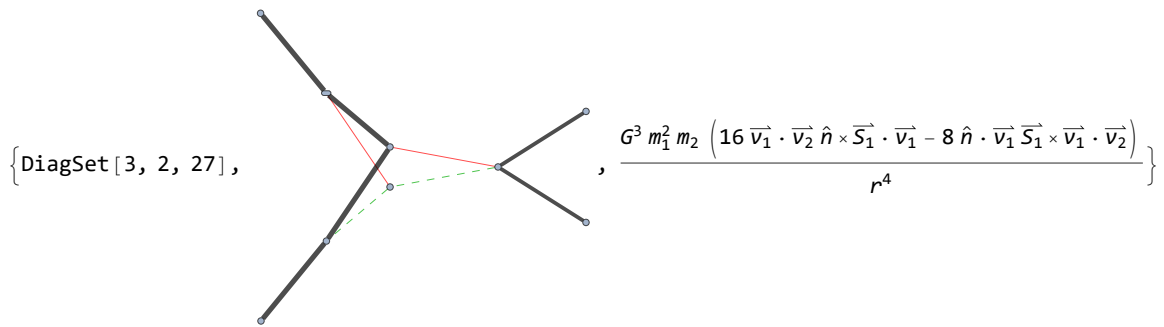

$$\left\{ \text{DiagSet}[3, 2, 28], \right. , \left. \frac{G^3 m_1^2 m_2 \left( \hat{n} \cdot \vec{v}_1 \hat{n} \times \vec{S}_1 \cdot \vec{v}_1 - \hat{n} \cdot \vec{v}_1 \hat{n} \times \vec{a}_1 \cdot \vec{S}_1 \right)}{r^3} + \right.$$
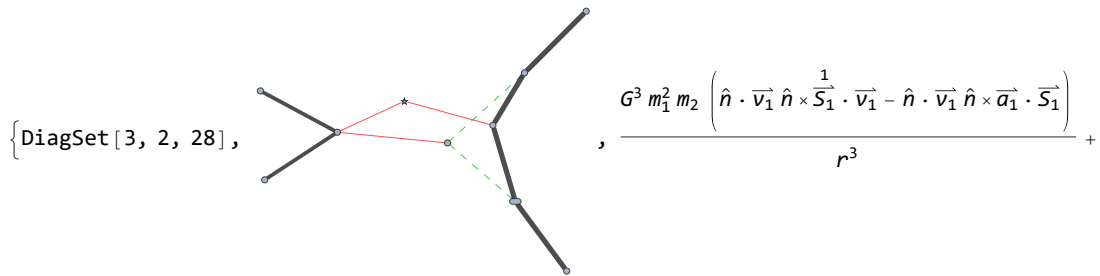

$$\left. \frac{1}{r^4} G^3 m_1^2 m_2 \left( -4 \left( \hat{n} \cdot \vec{v}_1 \right)^2 \hat{n} \times \vec{S}_1 \cdot \vec{v}_1 - \hat{n} \cdot \vec{v}_1 \vec{S}_1 \times \vec{v}_1 \cdot \vec{v}_2 + 5 \hat{n} \cdot \vec{v}_2 \hat{n} \cdot \vec{v}_1 \hat{n} \times \vec{S}_1 \cdot \vec{v}_1 - \vec{v}_1 \cdot \vec{v}_2 \hat{n} \times \vec{S}_1 \cdot \vec{v}_1 \right) \right\}$$

$$\left\{ \text{DiagSet}[3, 2, 29], \right. ,$$
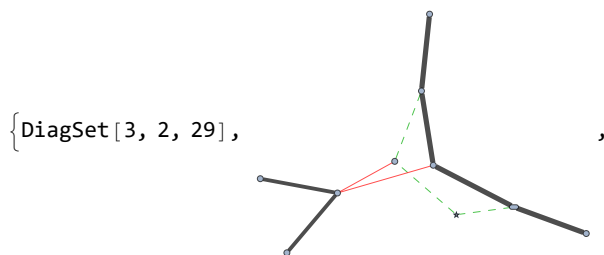

$$\frac{1}{r^3} G^3 m_1^2 m_2 \left( \hat{n} \cdot \vec{a}_1 \hat{n} \times \vec{S}_1 \cdot \vec{v}_1 + \vec{a}_1 \times \vec{S}_1 \cdot \vec{v}_1 + 5 \hat{n} \cdot \vec{v}_1 \hat{n} \times \vec{S}_1 \cdot \vec{v}_1 - 6 \hat{n} \cdot \vec{v}_2 \hat{n} \times \vec{S}_1 \cdot \vec{v}_1 + 2 \vec{S}_1 \times \vec{v}_1 \cdot \vec{v}_2 \right) + \frac{2 G^3 m_1^2 m_2 \hat{n} \times \vec{a}_1 \cdot \vec{S}_1}{r^2} +$$

$$\frac{1}{r^4} G^3 m_1^2 m_2 \left( -3 \left( \hat{n} \cdot \vec{v}_1 \right)^2 \hat{n} \times \vec{S}_1 \cdot \vec{v}_1 - \hat{n} \cdot \vec{v}_1 \vec{S}_1 \times \vec{v}_1 \cdot \vec{v}_2 + 5 \hat{n} \cdot \vec{v}_2 \hat{n} \cdot \vec{v}_1 \hat{n} \times \vec{S}_1 \cdot \vec{v}_1 + \vec{v}_1 \cdot \vec{v}_2 \hat{n} \times \vec{S}_1 \cdot \vec{v}_1 - \vec{v}_1 \cdot \vec{v}_2 \hat{n} \times \vec{S}_1 \cdot \vec{v}_1 \right) \left\}$$

$$\left\{ \text{DiagSet}[3, 2, 30], \right. ,$$
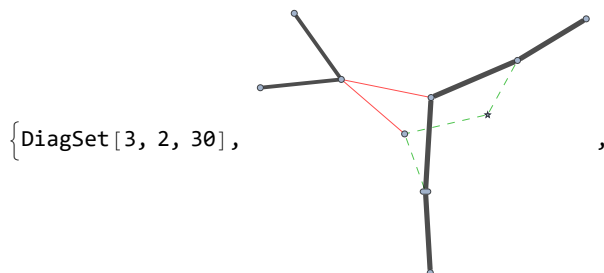

$$\frac{1}{r^3} G^3 m_1^2 m_2 \left( 3 \hat{n} \cdot \vec{a}_1 \hat{n} \times \vec{S}_1 \cdot \vec{v}_1 + 8 \hat{n} \cdot \vec{v}_1 \hat{n} \times \vec{a}_1 \cdot \vec{S}_1 - 6 \hat{n} \cdot \vec{v}_2 \hat{n} \times \vec{a}_1 \cdot \vec{S}_1 - 3 \vec{a}_1 \times \vec{S}_1 \cdot \vec{v}_1 + 2 \vec{a}_1 \times \vec{S}_1 \cdot \vec{v}_2 - \hat{n} \cdot \vec{v}_1 \hat{n} \times \vec{S}_1 \cdot \vec{v}_1 \right) -$$

$$\frac{2 G^3 m_1^2 m_2 \hat{n} \times \vec{a}_1 \cdot \vec{S}_1}{r^2} + \frac{1}{r^4}$$

$$G^3 m_1^2 m_2 \left( 3 \left( \hat{n} \cdot \vec{v}_1 \right)^2 \hat{n} \times \vec{S}_1 \cdot \vec{v}_1 + \hat{n} \cdot \vec{v}_1 \vec{S}_1 \times \vec{v}_1 \cdot \vec{v}_2 - 5 \hat{n} \cdot \vec{v}_2 \hat{n} \cdot \vec{v}_1 \hat{n} \times \vec{S}_1 \cdot \vec{v}_1 - \vec{v}_1 \cdot \vec{v}_2 \hat{n} \times \vec{S}_1 \cdot \vec{v}_1 + \vec{v}_1 \cdot \vec{v}_2 \hat{n} \times \vec{S}_1 \cdot \vec{v}_1 \right) \left\}$$



$\{\text{DiagSet}[3, 2, 31],$  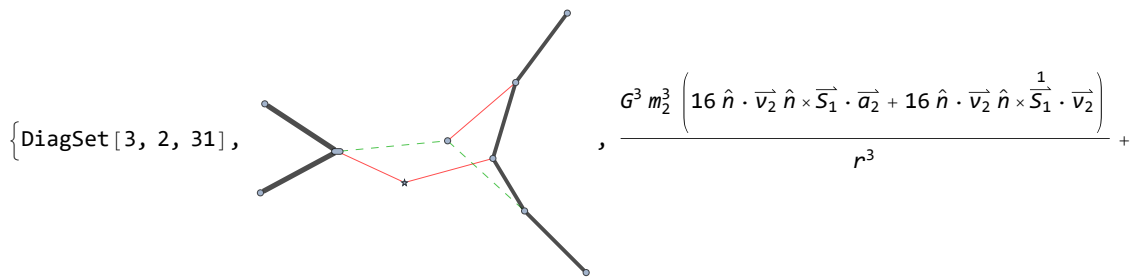 ,  $\frac{G^3 m_2^3 \left( 16 \hat{n} \cdot \vec{v}_2 \hat{n} \times \vec{S}_1 \cdot \vec{a}_2 + 16 \hat{n} \cdot \vec{v}_2 \hat{n} \times \vec{S}_1 \cdot \vec{v}_2 \right)}{r^3} +$

$$\frac{1}{r^4} G^3 m_2^3 \left( 64 (\hat{n} \cdot \vec{v}_2)^2 \hat{n} \times \vec{S}_1 \cdot \vec{v}_2 - 16 \hat{n} \cdot \vec{v}_2 \vec{S}_1 \times \vec{v}_1 \cdot \vec{v}_2 - 80 \hat{n} \cdot \vec{v}_1 \hat{n} \cdot \vec{v}_2 \hat{n} \times \vec{S}_1 \cdot \vec{v}_2 + 16 \vec{v}_1 \cdot \vec{v}_2 \hat{n} \times \vec{S}_1 \cdot \vec{v}_2 \right) \}$$

$\{\text{DiagSet}[3, 2, 32],$  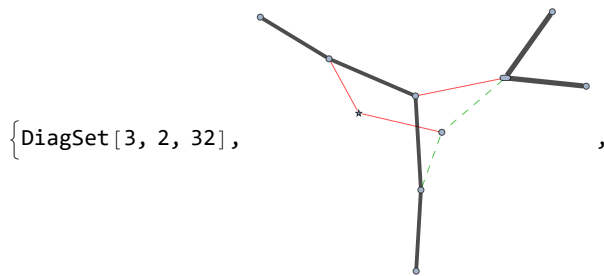 ,

$$\frac{G^3 m_2^3 \left( 16 \hat{n} \cdot \vec{a}_2 \hat{n} \times \vec{S}_1 \cdot \vec{v}_2 - 8 \vec{S}_1 \times \vec{v}_2 \cdot \vec{a}_2 + 16 \hat{n} \cdot \vec{v}_2 \hat{n} \times \vec{S}_1 \cdot \vec{v}_2 \right)}{r^3} + \frac{1}{r^4}$$

$$G^3 m_2^3 \left( 64 (\hat{n} \cdot \vec{v}_2)^2 \hat{n} \times \vec{S}_1 \cdot \vec{v}_2 - 16 \hat{n} \cdot \vec{v}_2 \vec{S}_1 \times \vec{v}_1 \cdot \vec{v}_2 - 80 \hat{n} \cdot \vec{v}_1 \hat{n} \cdot \vec{v}_2 \hat{n} \times \vec{S}_1 \cdot \vec{v}_2 + 16 \vec{v}_1 \cdot \vec{v}_2 \hat{n} \times \vec{S}_1 \cdot \vec{v}_2 \right) \}$$

$\{\text{DiagSet}[3, 2, 33],$  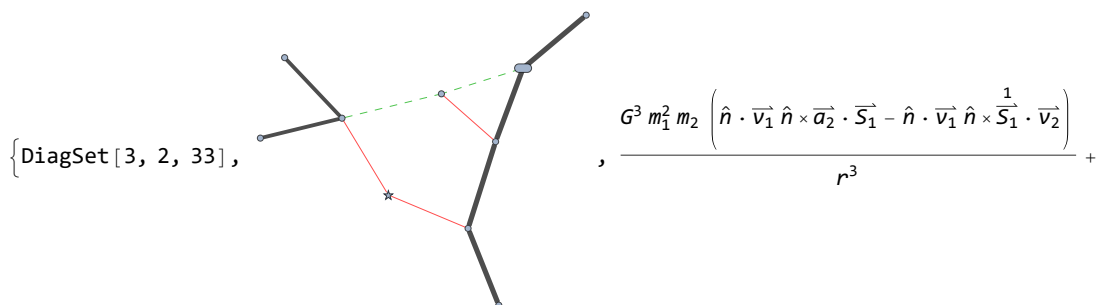 ,  $\frac{G^3 m_1^2 m_2 \left( \hat{n} \cdot \vec{v}_1 \hat{n} \times \vec{a}_2 \cdot \vec{S}_1 - \hat{n} \cdot \vec{v}_1 \hat{n} \times \vec{S}_1 \cdot \vec{v}_2 \right)}{r^3} +$

$$\frac{1}{r^4} G^3 m_1^2 m_2 \left( 4 (\hat{n} \cdot \vec{v}_1)^2 \hat{n} \times \vec{S}_1 \cdot \vec{v}_2 + \hat{n} \cdot \vec{v}_1 \vec{S}_1 \times \vec{v}_1 \cdot \vec{v}_2 - 5 \hat{n} \cdot \vec{v}_2 \hat{n} \cdot \vec{v}_1 \hat{n} \times \vec{S}_1 \cdot \vec{v}_2 + \vec{v}_1 \cdot \vec{v}_2 \hat{n} \times \vec{S}_1 \cdot \vec{v}_2 \right) \}$$

$\{\text{DiagSet}[3, 2, 34],$  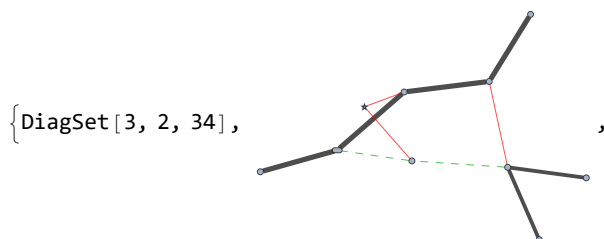 ,

$$\frac{1}{r^3} G^3 m_1^2 m_2 \left( 3 \hat{n} \cdot \vec{a}_2 \hat{n} \times \vec{S}_1 \cdot \vec{v}_1 + 2 \hat{n} \cdot \vec{v}_1 \hat{n} \times \vec{a}_2 \cdot \vec{S}_1 - \vec{a}_2 \times \vec{S}_1 \cdot \vec{v}_1 - 2 \hat{n} \cdot \vec{v}_1 \hat{n} \times \vec{S}_1 \cdot \vec{v}_2 + 3 \hat{n} \cdot \vec{v}_2 \hat{n} \times \vec{S}_1 \cdot \vec{v}_1 - \left( \vec{S}_1 \times \vec{v}_1 \cdot \vec{v}_2 \right) \right) +$$

$$\frac{1}{r^4} G^3 m_1^2 m_2 \left( 8 (\hat{n} \cdot \vec{v}_1)^2 \hat{n} \times \vec{S}_1 \cdot \vec{v}_2 + 5 \hat{n} \cdot \vec{v}_1 \vec{S}_1 \times \vec{v}_1 \cdot \vec{v}_2 - 11 \hat{n} \cdot \vec{v}_2 \hat{n} \cdot \vec{v}_1 \hat{n} \times \vec{S}_1 \cdot \vec{v}_1 - 10 \hat{n} \cdot \vec{v}_2 \hat{n} \cdot \vec{v}_1 \hat{n} \times \vec{S}_1 \cdot \vec{v}_2 + \right. \\ \left. 15 (\hat{n} \cdot \vec{v}_2)^2 \hat{n} \times \vec{S}_1 \cdot \vec{v}_1 - 6 \hat{n} \cdot \vec{v}_2 \vec{S}_1 \times \vec{v}_1 \cdot \vec{v}_2 + \vec{v}_1 \cdot \vec{v}_2 \hat{n} \times \vec{S}_1 \cdot \vec{v}_1 + 2 \vec{v}_1 \cdot \vec{v}_2 \hat{n} \times \vec{S}_1 \cdot \vec{v}_2 - 3 \vec{v}_2 \cdot \vec{v}_2 \hat{n} \times \vec{S}_1 \cdot \vec{v}_1 \right) \}$$

{DiagSet[3, 2, 35],

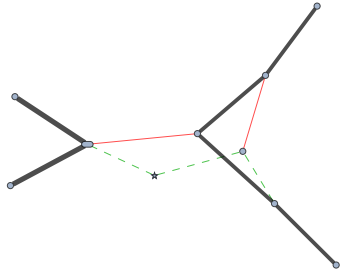

,

$$\frac{1}{r^3} G^3 m_2^3 \left( -48 \hat{n} \cdot \vec{v}_1 \hat{n} \times \vec{S}_1 \cdot \vec{a}_2 + 16 \hat{n} \cdot \vec{v}_2 \hat{n} \times \vec{S}_1 \cdot \vec{a}_2 - 16 \vec{S}_1 \times \vec{v}_1 \cdot \vec{a}_2 + 32 \hat{n} \cdot \vec{v}_2 \hat{n} \times \vec{S}_1 \cdot \vec{v}_2 \right) + \frac{16 G^3 m_2^3 \hat{n} \times \vec{S}_1 \cdot \vec{a}_2}{r^2} +$$

$$\frac{1}{r^4} G^3 m_2^3 \left( 32 (\hat{n} \cdot \vec{v}_2)^2 \hat{n} \times \vec{S}_1 \cdot \vec{v}_2 - 32 \hat{n} \cdot \vec{v}_2 \vec{S}_1 \times \vec{v}_1 \cdot \vec{v}_2 - 160 \hat{n} \cdot \vec{v}_1 \hat{n} \cdot \vec{v}_2 \hat{n} \times \vec{S}_1 \cdot \vec{v}_2 + 32 \vec{v}_1 \cdot \vec{v}_2 \hat{n} \times \vec{S}_1 \cdot \vec{v}_2 \right) \}$$

{DiagSet[3, 2, 36],

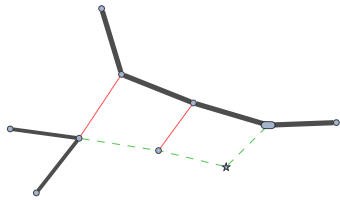

,

$$\frac{1}{r^3} G^3 m_1^2 m_2 \left( -\hat{n} \cdot \vec{a}_2 \hat{n} \times \vec{S}_1 \cdot \vec{v}_1 + 6 \hat{n} \cdot \vec{v}_1 \hat{n} \times \vec{a}_2 \cdot \vec{S}_1 - 3 \vec{a}_2 \times \vec{S}_1 \cdot \vec{v}_1 - 12 \hat{n} \cdot \vec{v}_1 \hat{n} \times \vec{S}_1 \cdot \vec{v}_2 + \right.$$

$$\left. \hat{n} \cdot \vec{v}_2 \hat{n} \times \vec{S}_1 \cdot \vec{v}_1 + 18 \hat{n} \cdot \vec{v}_2 \hat{n} \times \vec{S}_1 \cdot \vec{v}_2 - 3 \vec{S}_1 \times \vec{v}_1 \cdot \vec{v}_2 \right) - \frac{6 G^3 m_1^2 m_2 \hat{n} \times \vec{a}_2 \cdot \vec{S}_1}{r^2} + \frac{1}{r^4}$$

$$G^3 m_1^2 m_2 \left( 12 (\hat{n} \cdot \vec{v}_1)^2 \hat{n} \times \vec{S}_1 \cdot \vec{v}_2 + 7 \hat{n} \cdot \vec{v}_1 \vec{S}_1 \times \vec{v}_1 \cdot \vec{v}_2 + \hat{n} \cdot \vec{v}_2 \hat{n} \cdot \vec{v}_1 \hat{n} \times \vec{S}_1 \cdot \vec{v}_1 - 30 \hat{n} \cdot \vec{v}_2 \hat{n} \cdot \vec{v}_1 \hat{n} \times \vec{S}_1 \cdot \vec{v}_2 - 5 (\hat{n} \cdot \vec{v}_2)^2 \right.$$

$$\left. \hat{n} \times \vec{S}_1 \cdot \vec{v}_1 - 8 \hat{n} \cdot \vec{v}_2 \vec{S}_1 \times \vec{v}_1 \cdot \vec{v}_2 - 2 \vec{v}_1 \cdot \vec{v}_1 \hat{n} \times \vec{S}_1 \cdot \vec{v}_2 - \vec{v}_1 \cdot \vec{v}_2 \hat{n} \times \vec{S}_1 \cdot \vec{v}_1 + 6 \vec{v}_1 \cdot \vec{v}_2 \hat{n} \times \vec{S}_1 \cdot \vec{v}_2 + \vec{v}_2 \cdot \vec{v}_2 \hat{n} \times \vec{S}_1 \cdot \vec{v}_1 \right) \}$$

{DiagSet[3, 2, 37],

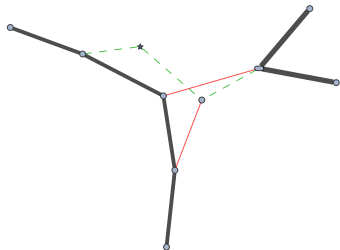

,

$$\frac{1}{r^3} G^3 m_2^3 \left( 16 \hat{n} \cdot \vec{a}_2 \hat{n} \times \vec{S}_1 \cdot \vec{v}_2 - 48 \hat{n} \cdot \vec{v}_1 \hat{n} \times \vec{S}_1 \cdot \vec{a}_2 + 16 \hat{n} \cdot \vec{v}_2 \hat{n} \times \vec{S}_1 \cdot \vec{a}_2 - \right.$$

$$\left. 16 \vec{S}_1 \times \vec{v}_1 \cdot \vec{a}_2 - 8 \vec{S}_1 \times \vec{v}_2 \cdot \vec{a}_2 + 16 \hat{n} \cdot \vec{v}_2 \hat{n} \times \vec{S}_1 \cdot \vec{v}_2 \right) + \frac{16 G^3 m_2^3 \hat{n} \times \vec{S}_1 \cdot \vec{a}_2}{r^2} + \frac{1}{r^4}$$

$$G^3 m_2^3 \left( 32 (\hat{n} \cdot \vec{v}_2)^2 \hat{n} \times \vec{S}_1 \cdot \vec{v}_2 - 16 \hat{n} \cdot \vec{v}_2 \vec{S}_1 \times \vec{v}_1 \cdot \vec{v}_2 - 80 \hat{n} \cdot \vec{v}_1 \hat{n} \cdot \vec{v}_2 \hat{n} \times \vec{S}_1 \cdot \vec{v}_2 + 16 \vec{v}_1 \cdot \vec{v}_2 \hat{n} \times \vec{S}_1 \cdot \vec{v}_2 \right) \}$$

{DiagSet[3, 2, 38],

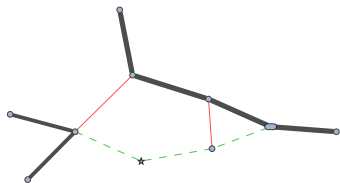

,

$$\frac{G^3 m_1^2 m_2 \left( 2 \hat{n} \cdot \vec{v}_1 \hat{n} \times \vec{a}_2 \cdot \vec{S}_1 - (\vec{a}_2 \times \vec{S}_1 \cdot \vec{v}_1) - \hat{n} \cdot \vec{v}_1 \hat{n} \times \vec{S}_1 \cdot \vec{v}_2 + 3 \hat{n} \cdot \vec{v}_2 \hat{n} \times \vec{S}_1 \cdot \vec{v}_2 \right)}{r^3} - \frac{G^3 m_1^2 m_2 \hat{n} \times \vec{a}_2 \cdot \vec{S}_1}{r^2} + \frac{1}{r^4}$$

$$G^3 m_1^2 m_2 \left( 2 \left( \hat{n} \cdot \vec{v}_1 \right)^2 \hat{n} \times \vec{S}_1 \cdot \vec{v}_2 + \hat{n} \cdot \vec{v}_1 \vec{S}_1 \times \vec{v}_1 \cdot \vec{v}_2 - 10 \hat{n} \cdot \vec{v}_2 \hat{n} \cdot \vec{v}_1 \hat{n} \times \vec{S}_1 \cdot \vec{v}_2 - 3 \hat{n} \cdot \vec{v}_2 \vec{S}_1 \times \vec{v}_1 \cdot \vec{v}_2 + 2 \vec{v}_1 \cdot \vec{v}_2 \hat{n} \times \vec{S}_1 \cdot \vec{v}_2 \right) \Big\}$$

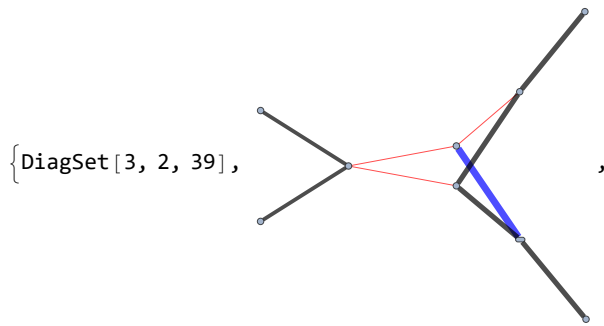

$$\frac{1}{r^3} G^3 m_1^2 m_2 \left( -4 \hat{n} \cdot \vec{a}_1 \hat{n} \times \vec{S}_1 \cdot \vec{v}_1 + 8 \hat{n} \cdot \vec{v}_1 \hat{n} \times \vec{a}_1 \cdot \vec{S}_1 - 2 \vec{a}_1 \times \vec{S}_1 \cdot \vec{v}_1 - 6 \hat{n} \cdot \vec{v}_1 \hat{n} \times \vec{S}_1 \cdot \vec{v}_1 \right) +$$

$$\frac{1}{r^4} G^3 m_1^2 m_2 \left( 5 \left( \hat{n} \cdot \vec{v}_1 \right)^2 \hat{n} \times \vec{S}_1 \cdot \vec{v}_1 + \hat{n} \cdot \vec{v}_1 \vec{S}_1 \times \vec{v}_1 \cdot \vec{v}_2 - \right.$$

$$\left. 5 \hat{n} \cdot \vec{v}_2 \hat{n} \cdot \vec{v}_1 \hat{n} \times \vec{S}_1 \cdot \vec{v}_1 + \frac{1}{4} \vec{v}_1 \cdot \vec{v}_1 \hat{n} \times \vec{S}_1 \cdot \vec{v}_1 + \vec{v}_1 \cdot \vec{v}_2 \hat{n} \times \vec{S}_1 \cdot \vec{v}_1 - \frac{9}{4} \vec{v}_2 \cdot \vec{v}_2 \hat{n} \times \vec{S}_1 \cdot \vec{v}_1 \right) \Big\}$$

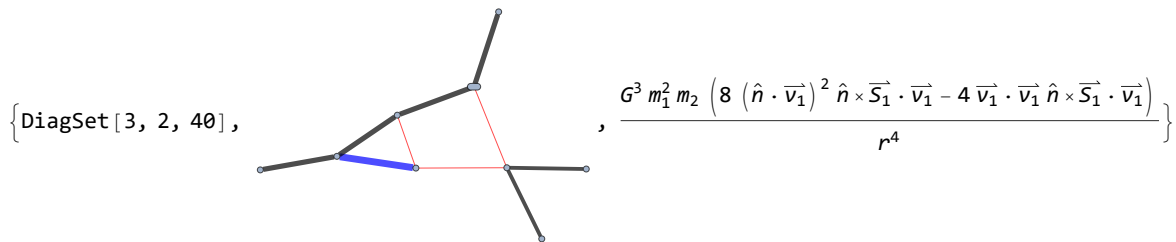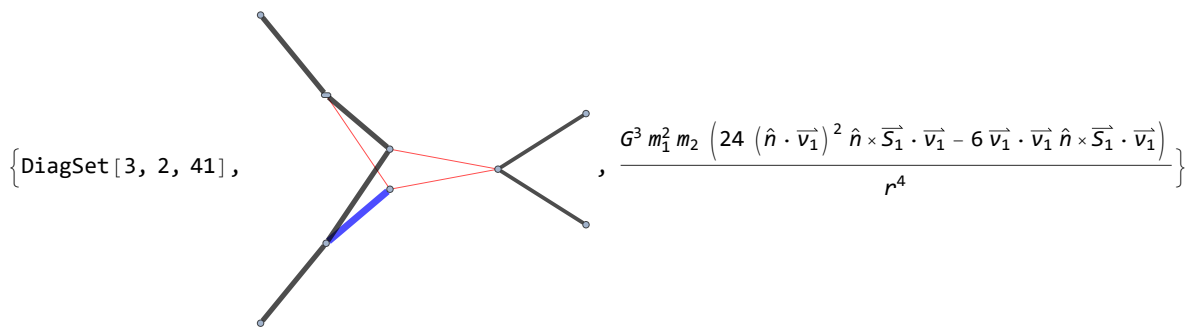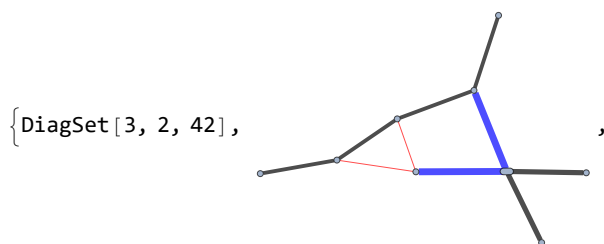

$$\frac{G^3 m_2^3 \left( -\frac{1}{2} \hat{n} \cdot \vec{a}_2 \hat{n} \times \vec{S}_1 \cdot \vec{v}_2 - \frac{1}{2} \hat{n} \cdot \vec{v}_2 \hat{n} \times \vec{S}_1 \cdot \vec{a}_2 \right)}{r^3} + \frac{1}{r^4} G^3 m_2^3 \left( \frac{3}{2} \left( \hat{n} \cdot \vec{v}_2 \right)^2 \hat{n} \times \vec{S}_1 \cdot \vec{v}_2 + \frac{1}{2} \hat{n} \cdot \vec{v}_2 \vec{S}_1 \times \vec{v}_1 \cdot \vec{v}_2 - \right.$$

$$\left. \frac{3}{2} \hat{n} \cdot \vec{v}_1 \hat{n} \cdot \vec{v}_2 \hat{n} \times \vec{S}_1 \cdot \vec{v}_2 + \frac{5}{2} \vec{v}_1 \cdot \vec{v}_2 \hat{n} \times \vec{S}_1 \cdot \vec{v}_2 - 3 \vec{v}_2 \cdot \vec{v}_2 \hat{n} \times \vec{S}_1 \cdot \vec{v}_1 - \frac{1}{2} \vec{v}_2 \cdot \vec{v}_2 \hat{n} \times \vec{S}_1 \cdot \vec{v}_2 \right) \Big\}$$

$\{\text{DiagSet}[3, 2, 43],$ 
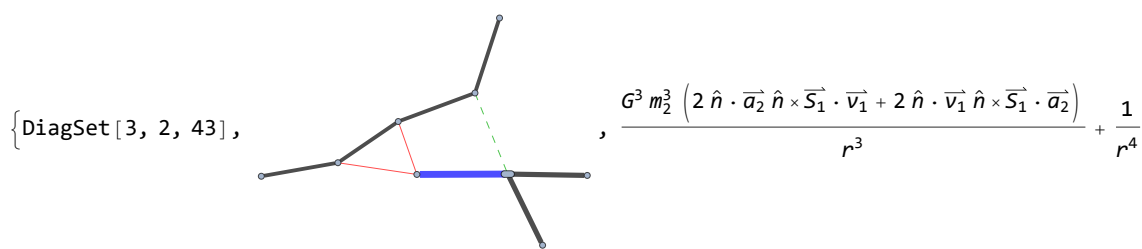
 $, \frac{G^3 m_2^3 \left( 2 \hat{n} \cdot \vec{a}_2 \hat{n} \times \vec{S}_1 \cdot \vec{v}_1 + 2 \hat{n} \cdot \vec{v}_1 \hat{n} \times \vec{S}_1 \cdot \vec{a}_2 \right)}{r^3} + \frac{1}{r^4}$

$$G^3 m_2^3 \left\{ -\frac{3}{2} (\hat{n} \cdot \vec{v}_1)^2 \hat{n} \times \vec{S}_1 \cdot \vec{v}_2 - \frac{3}{2} \hat{n} \cdot \vec{v}_2 \hat{n} \cdot \vec{v}_1 \hat{n} \times \vec{S}_1 \cdot \vec{v}_1 - 6 \hat{n} \cdot \vec{v}_2 \hat{n} \cdot \vec{v}_1 \hat{n} \times \vec{S}_1 \cdot \vec{v}_2 + 2 (\hat{n} \cdot \vec{v}_2)^2 \hat{n} \times \vec{S}_1 \cdot \vec{v}_1 - \right.$$

$$\left. 2 (\hat{n} \cdot \vec{v}_2)^2 \hat{n} \times \vec{S}_1 \cdot \vec{v}_2 - 4 \hat{n} \cdot \vec{v}_2 \vec{S}_1 \times \vec{v}_1 \cdot \vec{v}_2 + \frac{3}{2} \vec{v}_1 \cdot \vec{v}_2 \hat{n} \times \vec{S}_1 \cdot \vec{v}_1 + 2 \vec{v}_1 \cdot \vec{v}_2 \hat{n} \times \vec{S}_1 \cdot \vec{v}_2 - \frac{3}{2} \vec{v}_2 \cdot \vec{v}_2 \hat{n} \times \vec{S}_1 \cdot \vec{v}_1 \right\}$$

$\{\text{DiagSet}[3, 2, 44],$ 
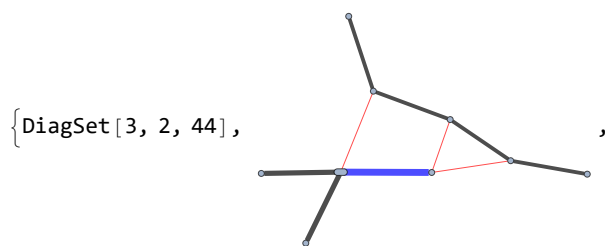
 $,$

$$\frac{G^3 m_2^3 \left( \hat{n} \cdot \vec{a}_1 \hat{n} \times \vec{S}_1 \cdot \vec{v}_1 - \hat{n} \cdot \vec{v}_1 \hat{n} \times \vec{S}_1 \cdot \vec{a}_1 - 2 \vec{S}_1 \times \vec{v}_1 \cdot \vec{a}_1 \right)}{r^3} + \frac{1}{r^4} G^3 m_2^3 \left\{ -3 (\hat{n} \cdot \vec{v}_1)^2 \hat{n} \times \vec{S}_1 \cdot \vec{v}_1 - 3 \hat{n} \cdot \vec{v}_1 \vec{S}_1 \times \vec{v}_1 \cdot \vec{v}_2 + \right.$$

$$\left. 12 \hat{n} \cdot \vec{v}_2 \hat{n} \cdot \vec{v}_1 \hat{n} \times \vec{S}_1 \cdot \vec{v}_1 - \frac{3}{2} \vec{v}_1 \cdot \vec{v}_1 \hat{n} \times \vec{S}_1 \cdot \vec{v}_1 - 3 \vec{v}_1 \cdot \vec{v}_2 \hat{n} \times \vec{S}_1 \cdot \vec{v}_1 - \frac{9}{2} \vec{v}_2 \cdot \vec{v}_2 \hat{n} \times \vec{S}_1 \cdot \vec{v}_1 \right\}$$

$\{\text{DiagSet}[3, 2, 45],$ 
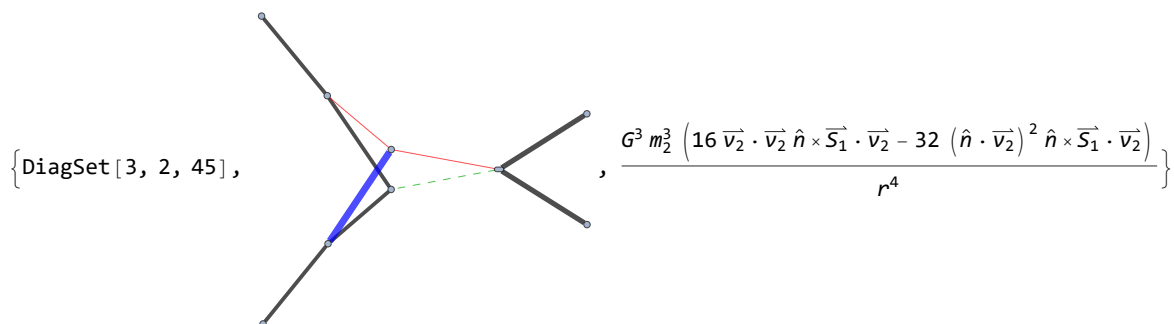
 $, \frac{G^3 m_2^3 \left( 16 \vec{v}_2 \cdot \vec{v}_2 \hat{n} \times \vec{S}_1 \cdot \vec{v}_2 - 32 (\hat{n} \cdot \vec{v}_2)^2 \hat{n} \times \vec{S}_1 \cdot \vec{v}_2 \right)}{r^4} \}$

$\{\text{DiagSet}[3, 2, 46],$ 
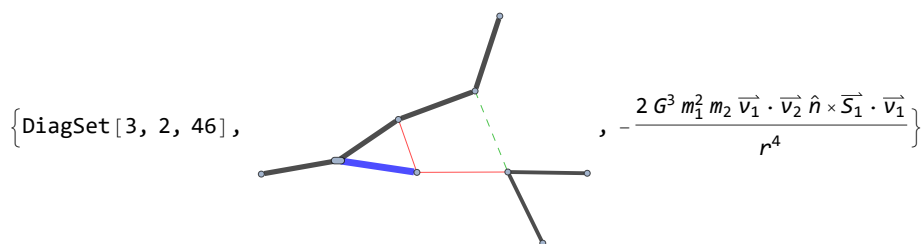
 $, -\frac{2 G^3 m_1^2 m_2 \vec{v}_1 \cdot \vec{v}_2 \hat{n} \times \vec{S}_1 \cdot \vec{v}_1}{r^4} \}$

$\{\text{DiagSet}[3, 2, 47],$ 
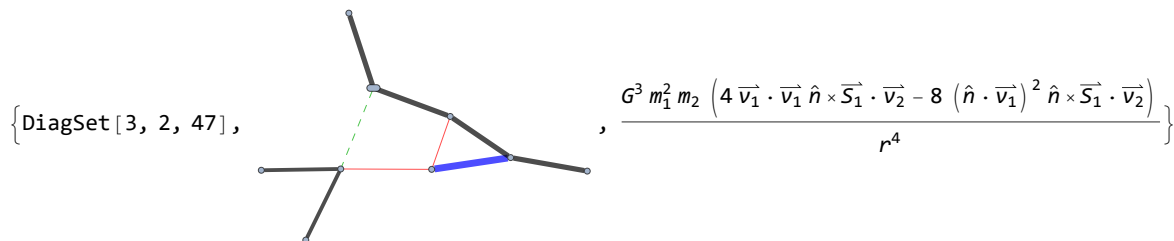
 $, \frac{G^3 m_1^2 m_2 \left( 4 \vec{v}_1 \cdot \vec{v}_1 \hat{n} \times \vec{S}_1 \cdot \vec{v}_2 - 8 (\hat{n} \cdot \vec{v}_1)^2 \hat{n} \times \vec{S}_1 \cdot \vec{v}_2 \right)}{r^4} \}$

$\{\text{DiagSet}[3, 2, 48],$

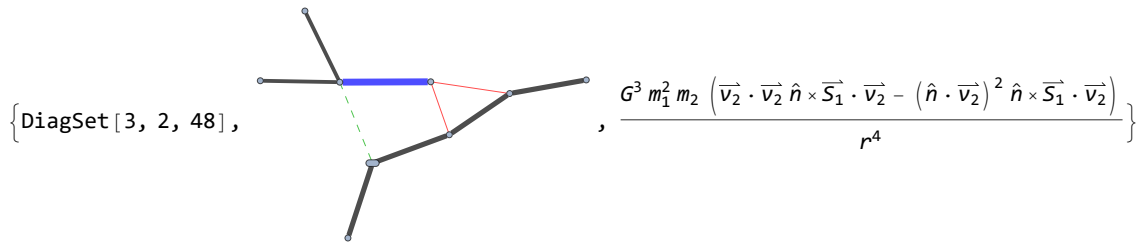

$, \frac{G^3 m_1^2 m_2 \left( \vec{v}_2 \cdot \vec{v}_2 \hat{n} \times \vec{S}_1 \cdot \vec{v}_2 - (\hat{n} \cdot \vec{v}_2)^2 \hat{n} \times \vec{S}_1 \cdot \vec{v}_2 \right)}{r^4} \}$

$\{\text{DiagSet}[3, 2, 49],$

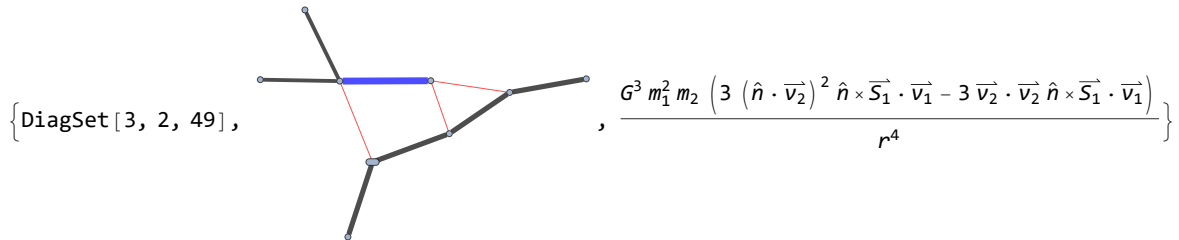

$, \frac{G^3 m_1^2 m_2 \left( 3 (\hat{n} \cdot \vec{v}_2)^2 \hat{n} \times \vec{S}_1 \cdot \vec{v}_1 - 3 \vec{v}_2 \cdot \vec{v}_2 \hat{n} \times \vec{S}_1 \cdot \vec{v}_1 \right)}{r^4} \}$

$\{\text{DiagSet}[3, 2, 50],$

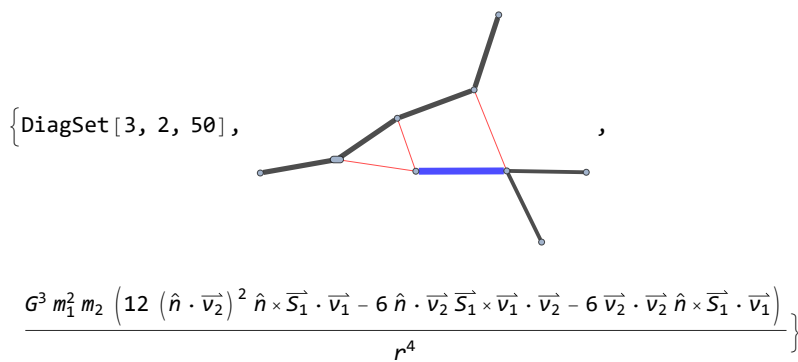

$, \frac{G^3 m_1^2 m_2 \left( 12 (\hat{n} \cdot \vec{v}_2)^2 \hat{n} \times \vec{S}_1 \cdot \vec{v}_1 - 6 \hat{n} \cdot \vec{v}_2 \vec{S}_1 \times \vec{v}_1 \cdot \vec{v}_2 - 6 \vec{v}_2 \cdot \vec{v}_2 \hat{n} \times \vec{S}_1 \cdot \vec{v}_1 \right)}{r^4} \}$

$\{\text{DiagSet}[3, 2, 51],$

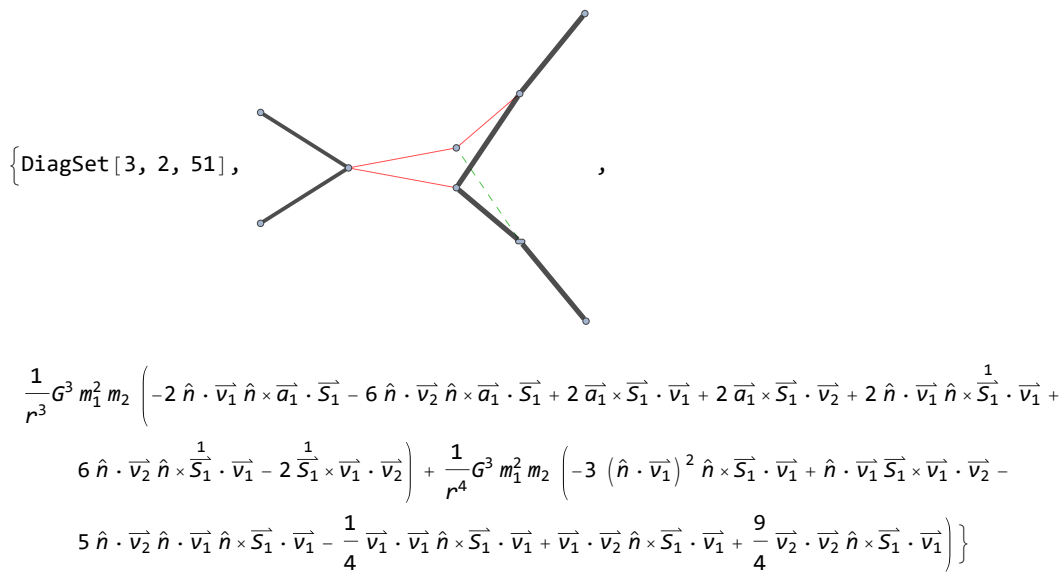

$, \frac{1}{r^3} G^3 m_1^2 m_2 \left( -2 \hat{n} \cdot \vec{v}_1 \hat{n} \times \vec{a}_1 \cdot \vec{S}_1 - 6 \hat{n} \cdot \vec{v}_2 \hat{n} \times \vec{a}_1 \cdot \vec{S}_1 + 2 \vec{a}_1 \times \vec{S}_1 \cdot \vec{v}_1 + 2 \vec{a}_1 \times \vec{S}_1 \cdot \vec{v}_2 + 2 \hat{n} \cdot \vec{v}_1 \hat{n} \times \vec{S}_1 \cdot \vec{v}_1 + \right.$   
 $6 \hat{n} \cdot \vec{v}_2 \hat{n} \times \vec{S}_1 \cdot \vec{v}_1 - 2 \vec{S}_1 \times \vec{v}_1 \cdot \vec{v}_2 \Big) + \frac{1}{r^4} G^3 m_1^2 m_2 \left( -3 (\hat{n} \cdot \vec{v}_1)^2 \hat{n} \times \vec{S}_1 \cdot \vec{v}_1 + \hat{n} \cdot \vec{v}_1 \vec{S}_1 \times \vec{v}_1 \cdot \vec{v}_2 - \right.$   
 $5 \hat{n} \cdot \vec{v}_2 \hat{n} \cdot \vec{v}_1 \hat{n} \times \vec{S}_1 \cdot \vec{v}_1 - \frac{1}{4} \vec{v}_1 \cdot \vec{v}_1 \hat{n} \times \vec{S}_1 \cdot \vec{v}_1 + \vec{v}_1 \cdot \vec{v}_2 \hat{n} \times \vec{S}_1 \cdot \vec{v}_1 + \frac{9}{4} \vec{v}_2 \cdot \vec{v}_2 \hat{n} \times \vec{S}_1 \cdot \vec{v}_1 \Big) \}$

$\{\text{DiagSet}[3, 2, 52],$

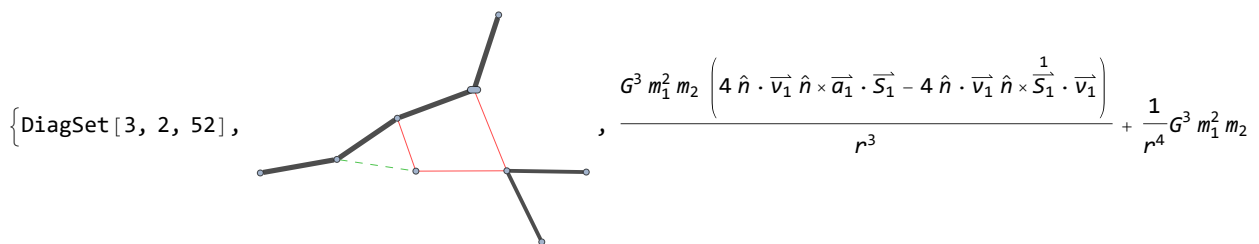

$, \frac{G^3 m_1^2 m_2 \left( 4 \hat{n} \cdot \vec{v}_1 \hat{n} \times \vec{a}_1 \cdot \vec{S}_1 - 4 \hat{n} \cdot \vec{v}_1 \hat{n} \times \vec{S}_1 \cdot \vec{v}_1 \right)}{r^3} + \frac{1}{r^4} G^3 m_1^2 m_2$

$\left( 4 (\hat{n} \cdot \vec{v}_1)^2 \hat{n} \times \vec{S}_1 \cdot \vec{v}_1 + 4 \hat{n} \cdot \vec{v}_1 \vec{S}_1 \times \vec{v}_1 \cdot \vec{v}_2 - 20 \hat{n} \cdot \vec{v}_2 \hat{n} \cdot \vec{v}_1 \hat{n} \times \vec{S}_1 \cdot \vec{v}_1 + 4 \vec{v}_1 \cdot \vec{v}_1 \hat{n} \times \vec{S}_1 \cdot \vec{v}_1 + 4 \vec{v}_1 \cdot \vec{v}_2 \hat{n} \times \vec{S}_1 \cdot \vec{v}_1 \right) \}$

{DiagSet[3, 2, 53],

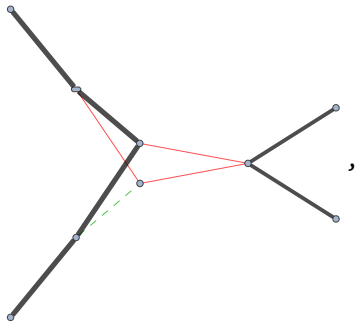

$$\frac{G^3 m_1^2 m_2 \left( -8 \hat{n} \cdot \vec{v}_1 \hat{n} \times \vec{a}_1 \cdot \vec{S}_1 + 4 \vec{a}_1 \times \vec{S}_1 \cdot \vec{v}_1 + 8 \hat{n} \cdot \vec{v}_1 \hat{n} \times \vec{S}_1 \cdot \vec{v}_1 \right)}{r^3} + \frac{1}{r^4} G^3 m_1^2 m_2$$

$$\left( -18 (\hat{n} \cdot \vec{v}_1)^2 \hat{n} \times \vec{S}_1 \cdot \vec{v}_1 + 6 \hat{n} \cdot \vec{v}_1 \vec{S}_1 \times \vec{v}_1 \cdot \vec{v}_2 - 30 \hat{n} \cdot \vec{v}_2 \hat{n} \cdot \vec{v}_1 \hat{n} \times \vec{S}_1 \cdot \vec{v}_1 + 6 \vec{v}_1 \cdot \vec{v}_1 \hat{n} \times \vec{S}_1 \cdot \vec{v}_1 + 6 \vec{v}_1 \cdot \vec{v}_2 \hat{n} \times \vec{S}_1 \cdot \vec{v}_1 \right) \}$$

{DiagSet[3, 2, 54],

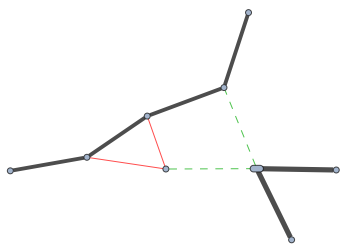

$$, \frac{G^3 m_2^3 \left( 2 \hat{n} \cdot \vec{a}_2 \hat{n} \times \vec{S}_1 \cdot \vec{v}_2 - 2 \hat{n} \cdot \vec{v}_2 \hat{n} \times \vec{S}_1 \cdot \vec{a}_2 - 4 \vec{S}_1 \times \vec{v}_2 \cdot \vec{a}_2 \right)}{r^3} +$$

$$\frac{1}{r^4} G^3 m_2^3 \left( 6 (\hat{n} \cdot \vec{v}_2)^2 \hat{n} \times \vec{S}_1 \cdot \vec{v}_2 - 2 \hat{n} \cdot \vec{v}_1 \hat{n} \cdot \vec{v}_2 \hat{n} \times \vec{S}_1 \cdot \vec{v}_2 + 4 \vec{v}_1 \cdot \vec{v}_2 \hat{n} \times \vec{S}_1 \cdot \vec{v}_2 - 2 \vec{v}_2 \cdot \vec{v}_2 \hat{n} \times \vec{S}_1 \cdot \vec{v}_2 \right) \}$$

{DiagSet[3, 2, 55],

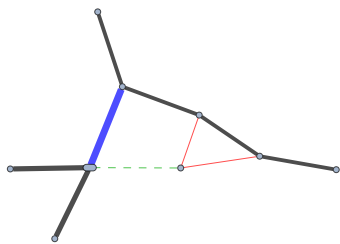

$$, \frac{G^3 m_2^3 \vec{v}_2 \cdot \vec{v}_2 \hat{n} \times \vec{S}_1 \cdot \vec{v}_2}{r^4} \}$$

{DiagSet[3, 2, 56],

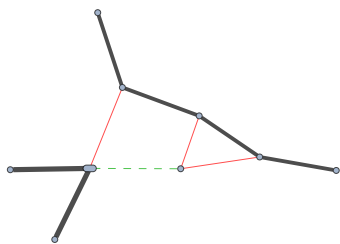

$$\frac{G^3 m_2^3 \left( 2 (\hat{n} \cdot \vec{v}_2)^2 \hat{n} \times \vec{S}_1 \cdot \vec{v}_1 - 2 \hat{n} \cdot \vec{v}_2 \vec{S}_1 \times \vec{v}_1 \cdot \vec{v}_2 - 9 \vec{v}_2 \cdot \vec{v}_2 \hat{n} \times \vec{S}_1 \cdot \vec{v}_2 \right)}{r^4} \}$$

{DiagSet[3, 2, 57],

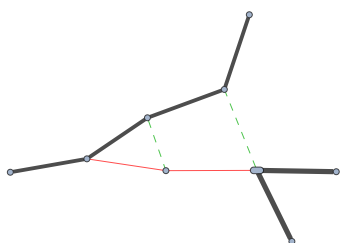

$$, \frac{G^3 m_2^3 \left( -16 \hat{n} \cdot \vec{v}_2 \hat{n} \times \vec{S}_1 \cdot \vec{a}_2 - 16 \hat{n} \cdot \vec{v}_2 \hat{n} \times \vec{S}_1 \cdot \vec{v}_2 \right)}{r^3} + \frac{1}{r^4} G^3 m_2^3$$

$$\left( -16 \left( \hat{n} \cdot \vec{v}_2 \right)^2 \hat{n} \times \vec{S}_1 \cdot \vec{v}_2 + 16 \hat{n} \cdot \vec{v}_2 \vec{S}_1 \times \vec{v}_1 \cdot \vec{v}_2 + 80 \hat{n} \cdot \vec{v}_1 \hat{n} \cdot \vec{v}_2 \hat{n} \times \vec{S}_1 \cdot \vec{v}_2 - 16 \vec{v}_1 \cdot \vec{v}_2 \hat{n} \times \vec{S}_1 \cdot \vec{v}_2 - 16 \vec{v}_2 \cdot \vec{v}_2 \hat{n} \times \vec{S}_1 \cdot \vec{v}_2 \right) \}$$

{DiagSet[3, 2, 58],

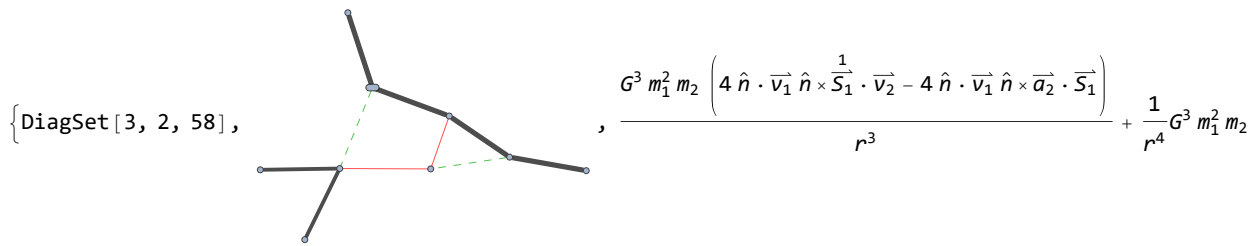

,  $\frac{G^3 m_1^2 m_2 \left( 4 \hat{n} \cdot \vec{v}_1 \hat{n} \times \vec{S}_1 \cdot \vec{v}_2 - 4 \hat{n} \cdot \vec{v}_1 \hat{n} \times \vec{a}_2 \cdot \vec{S}_1 \right)}{r^3} + \frac{1}{r^4} G^3 m_1^2 m_2$

$$\left( -4 \left( \hat{n} \cdot \vec{v}_1 \right)^2 \hat{n} \times \vec{S}_1 \cdot \vec{v}_2 - 4 \hat{n} \cdot \vec{v}_1 \vec{S}_1 \times \vec{v}_1 \cdot \vec{v}_2 + 20 \hat{n} \cdot \vec{v}_2 \hat{n} \cdot \vec{v}_1 \hat{n} \times \vec{S}_1 \cdot \vec{v}_2 - 4 \vec{v}_1 \cdot \vec{v}_1 \hat{n} \times \vec{S}_1 \cdot \vec{v}_2 - 4 \vec{v}_1 \cdot \vec{v}_2 \hat{n} \times \vec{S}_1 \cdot \vec{v}_2 \right) \}$$

{DiagSet[3, 2, 59],

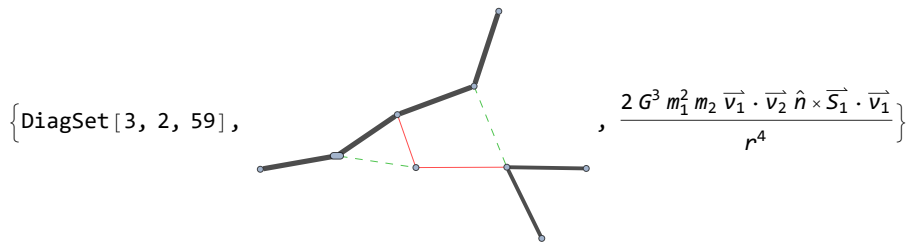

,  $\frac{2 G^3 m_1^2 m_2 \vec{v}_1 \cdot \vec{v}_2 \hat{n} \times \vec{S}_1 \cdot \vec{v}_1}{r^4} \}$

{DiagSet[3, 2, 60],

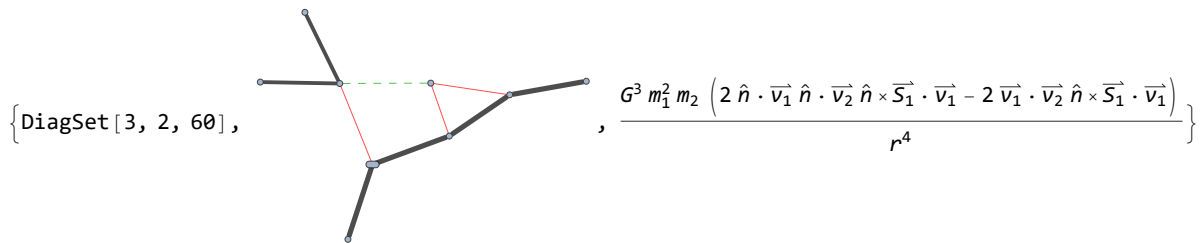

,  $\frac{G^3 m_1^2 m_2 \left( 2 \hat{n} \cdot \vec{v}_1 \hat{n} \cdot \vec{v}_2 \hat{n} \times \vec{S}_1 \cdot \vec{v}_1 - 2 \vec{v}_1 \cdot \vec{v}_2 \hat{n} \times \vec{S}_1 \cdot \vec{v}_1 \right)}{r^4} \}$

{DiagSet[3, 2, 61],

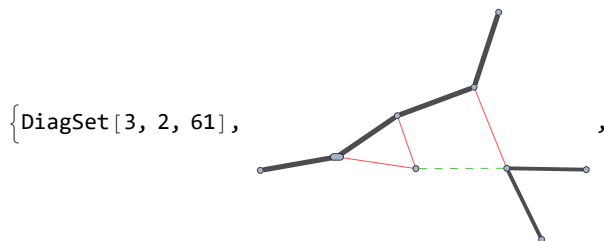

,

$$\frac{G^3 m_1^2 m_2 \left( 2 \hat{n} \cdot \vec{v}_2 \hat{n} \times \vec{a}_1 \cdot \vec{S}_1 - 2 \vec{a}_1 \times \vec{S}_1 \cdot \vec{v}_2 - 2 \hat{n} \cdot \vec{v}_2 \hat{n} \times \vec{S}_1 \cdot \vec{v}_1 + 2 \vec{S}_1 \times \vec{v}_1 \cdot \vec{v}_2 \right)}{r^3} +$$

$$\frac{G^3 m_1^2 m_2 \left( -2 \hat{n} \cdot \vec{v}_1 \vec{S}_1 \times \vec{v}_1 \cdot \vec{v}_2 + 8 \hat{n} \cdot \vec{v}_2 \hat{n} \cdot \vec{v}_1 \hat{n} \times \vec{S}_1 \cdot \vec{v}_1 - 4 \vec{v}_1 \cdot \vec{v}_2 \hat{n} \times \vec{S}_1 \cdot \vec{v}_1 \right)}{r^4} \}$$

{DiagSet[3, 2, 62],

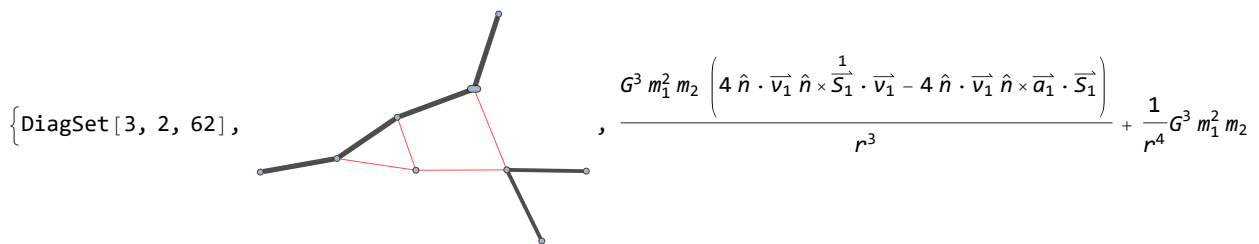

,  $\frac{G^3 m_1^2 m_2 \left( 4 \hat{n} \cdot \vec{v}_1 \hat{n} \times \vec{S}_1 \cdot \vec{v}_1 - 4 \hat{n} \cdot \vec{v}_1 \hat{n} \times \vec{a}_1 \cdot \vec{S}_1 \right)}{r^3} + \frac{1}{r^4} G^3 m_1^2 m_2$

$$\left( -13 \left( \hat{n} \cdot \vec{v}_1 \right)^2 \hat{n} \times \vec{S}_1 \cdot \vec{v}_1 - 4 \hat{n} \cdot \vec{v}_1 \vec{S}_1 \times \vec{v}_1 \cdot \vec{v}_2 + 20 \hat{n} \cdot \vec{v}_2 \hat{n} \cdot \vec{v}_1 \hat{n} \times \vec{S}_1 \cdot \vec{v}_1 + \vec{v}_1 \cdot \vec{v}_1 \hat{n} \times \vec{S}_1 \cdot \vec{v}_1 - 4 \vec{v}_1 \cdot \vec{v}_2 \hat{n} \times \vec{S}_1 \cdot \vec{v}_1 \right) \}$$

{DiagSet[3, 2, 63],

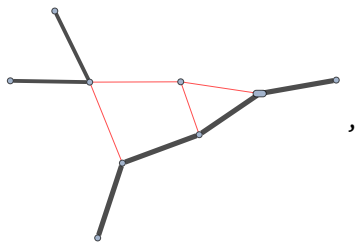

$$\frac{1}{r^3} G^3 m_1^2 m_2 \left( -6 \hat{n} \cdot \vec{v}_1 \hat{n} \times \vec{a}_1 \cdot \vec{S}_1 + 12 \hat{n} \cdot \vec{v}_2 \hat{n} \times \vec{a}_1 \cdot \vec{S}_1 + 2 \vec{a}_1 \times \vec{S}_1 \cdot \vec{v}_1 - \right. \\ \left. 4 \vec{a}_1 \times \vec{S}_1 \cdot \vec{v}_2 + 6 \hat{n} \cdot \vec{v}_1 \hat{n} \times \vec{S}_1 \cdot \vec{v}_1 - 12 \hat{n} \cdot \vec{v}_2 \hat{n} \times \vec{S}_1 \cdot \vec{v}_1 + 4 \vec{S}_1 \times \vec{v}_1 \cdot \vec{v}_2 \right) + \frac{1}{r^4} G^3 m_1^2 m_2 \\ \left( -12 (\hat{n} \cdot \vec{v}_1)^2 \hat{n} \times \vec{S}_1 \cdot \vec{v}_1 - 8 \hat{n} \cdot \vec{v}_1 \vec{S}_1 \times \vec{v}_1 \cdot \vec{v}_2 + 40 \hat{n} \cdot \vec{v}_2 \hat{n} \cdot \vec{v}_1 \hat{n} \times \vec{S}_1 \cdot \vec{v}_1 + 2 \vec{v}_1 \cdot \vec{v}_1 \hat{n} \times \vec{S}_1 \cdot \vec{v}_1 - 8 \vec{v}_1 \cdot \vec{v}_2 \hat{n} \times \vec{S}_1 \cdot \vec{v}_1 \right) \Big\}$$

{DiagSet[3, 2, 64],

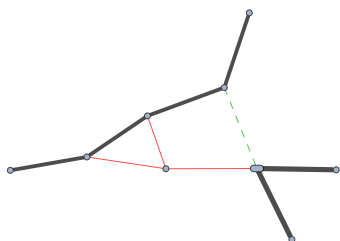

$$, \frac{G^3 m_2^3 \left( 16 \hat{n} \cdot \vec{v}_2 \hat{n} \times \vec{S}_1 \cdot \vec{a}_2 + 16 \hat{n} \cdot \vec{v}_2 \hat{n} \times \vec{S}_1 \cdot \vec{v}_2 \right)}{r^3} + \frac{1}{r^4} G^3 m_2^3$$

$$\left( 52 (\hat{n} \cdot \vec{v}_2)^2 \hat{n} \times \vec{S}_1 \cdot \vec{v}_2 - 16 \hat{n} \cdot \vec{v}_2 \vec{S}_1 \times \vec{v}_1 \cdot \vec{v}_2 - 80 \hat{n} \cdot \vec{v}_1 \hat{n} \cdot \vec{v}_2 \hat{n} \times \vec{S}_1 \cdot \vec{v}_2 + 16 \vec{v}_1 \cdot \vec{v}_2 \hat{n} \times \vec{S}_1 \cdot \vec{v}_2 - 4 \vec{v}_2 \cdot \vec{v}_2 \hat{n} \times \vec{S}_1 \cdot \vec{v}_2 \right) \Big\}$$

{DiagSet[3, 2, 65],

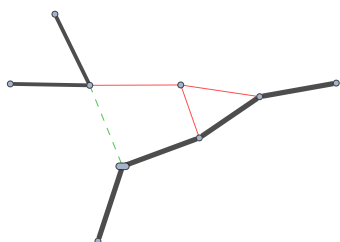

$$, \frac{G^3 m_1^2 m_2 \left( 4 \hat{n} \cdot \vec{v}_1 \hat{n} \times \vec{a}_2 \cdot \vec{S}_1 - 4 \hat{n} \cdot \vec{v}_1 \hat{n} \times \vec{S}_1 \cdot \vec{v}_2 \right)}{r^3} + \frac{1}{r^4}$$

$$G^3 m_1^2 m_2 \left( 13 (\hat{n} \cdot \vec{v}_1)^2 \hat{n} \times \vec{S}_1 \cdot \vec{v}_2 + 4 \hat{n} \cdot \vec{v}_1 \vec{S}_1 \times \vec{v}_1 \cdot \vec{v}_2 - 20 \hat{n} \cdot \vec{v}_2 \hat{n} \cdot \vec{v}_1 \hat{n} \times \vec{S}_1 \cdot \vec{v}_2 - \vec{v}_1 \cdot \vec{v}_1 \hat{n} \times \vec{S}_1 \cdot \vec{v}_2 + 4 \vec{v}_1 \cdot \vec{v}_2 \hat{n} \times \vec{S}_1 \cdot \vec{v}_2 \right) \Big\}$$

{DiagSet[3, 2, 66],

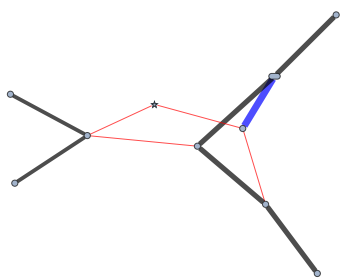

$$, \frac{1}{r^3} G^3 m_1^2 m_2$$

$$\left( \frac{1}{4} \hat{n} \cdot \vec{v}_1 \hat{n} \times \vec{a}_1 \cdot \vec{S}_1 - \frac{3}{4} \hat{n} \cdot \vec{v}_2 \hat{n} \times \vec{a}_1 \cdot \vec{S}_1 + \frac{1}{4} \vec{a}_1 \times \vec{S}_1 \cdot \vec{v}_2 - \frac{1}{4} \hat{n} \cdot \vec{v}_1 \hat{n} \times \vec{S}_1 \cdot \vec{v}_1 + \frac{3}{4} \hat{n} \cdot \vec{v}_2 \hat{n} \times \vec{S}_1 \cdot \vec{v}_1 - \frac{1}{4} \vec{S}_1 \times \vec{v}_1 \cdot \vec{v}_2 \right) + \\ \frac{1}{r^4} G^3 m_1^2 m_2 \left( \frac{1}{2} (\hat{n} \cdot \vec{v}_1)^2 \hat{n} \times \vec{S}_1 \cdot \vec{v}_1 + \frac{1}{2} \hat{n} \cdot \vec{v}_1 \vec{S}_1 \times \vec{v}_1 \cdot \vec{v}_2 - \frac{5}{2} \hat{n} \cdot \vec{v}_2 \hat{n} \cdot \vec{v}_1 \hat{n} \times \vec{S}_1 \cdot \vec{v}_1 + \frac{1}{2} \vec{v}_1 \cdot \vec{v}_2 \hat{n} \times \vec{S}_1 \cdot \vec{v}_1 \right) \Big\}$$



{DiagSet[3, 2, 67],

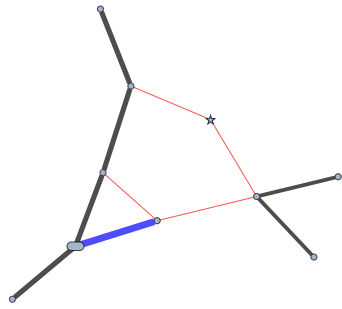

$$, \frac{G^3 m_1^2 m_2 \left( \frac{1}{4} \hat{n} \cdot \vec{v}_1 \hat{n} \times \vec{a}_1 \cdot \vec{S}_1 - \frac{1}{4} \hat{n} \cdot \vec{v}_1 \hat{n} \times \vec{S}_1 \cdot \vec{v}_1 \right)}{r^3} +$$

$$\frac{1}{r^4} G^3 m_1^2 m_2 \left( (\hat{n} \cdot \vec{v}_1)^2 \hat{n} \times \vec{S}_1 \cdot \vec{v}_1 + \frac{1}{4} \hat{n} \cdot \vec{v}_1 \vec{S}_1 \times \vec{v}_1 \cdot \vec{v}_2 - \frac{5}{4} \hat{n} \cdot \vec{v}_2 \hat{n} \cdot \vec{v}_1 \hat{n} \times \vec{S}_1 \cdot \vec{v}_1 + \frac{1}{4} \vec{v}_1 \cdot \vec{v}_2 \hat{n} \times \vec{S}_1 \cdot \vec{v}_1 \right) \}$$

{DiagSet[3, 2, 68],

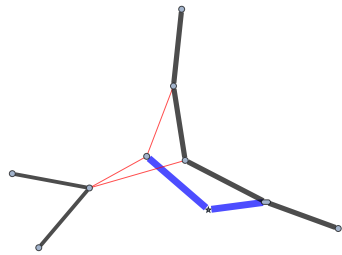

$$\frac{1}{r^3} G^3 m_1^2 m_2 \left( \frac{7}{4} \hat{n} \cdot \vec{a}_1 \hat{n} \times \vec{S}_1 \cdot \vec{v}_1 - \frac{5}{4} \hat{n} \cdot \vec{v}_1 \hat{n} \times \vec{a}_1 \cdot \vec{S}_1 + \frac{3}{2} \hat{n} \cdot \vec{v}_2 \hat{n} \times \vec{a}_1 \cdot \vec{S}_1 - \frac{1}{2} \vec{a}_1 \times \vec{S}_1 \cdot \vec{v}_1 - \frac{1}{2} \vec{a}_1 \times \vec{S}_1 \cdot \vec{v}_2 + 3 \hat{n} \cdot \vec{v}_1 \hat{n} \times \vec{S}_1 \cdot \vec{v}_1 - \frac{3}{2} \hat{n} \cdot \vec{v}_2 \hat{n} \times \vec{S}_1 \cdot \vec{v}_1 + \frac{1}{2} \vec{S}_1 \times \vec{v}_1 \cdot \vec{v}_2 \right) + \frac{1}{r^4} G^3 m_1^2 m_2 \left( 5 (\hat{n} \cdot \vec{v}_1)^2 \hat{n} \times \vec{S}_1 \cdot \vec{v}_1 + \frac{3}{2} \hat{n} \cdot \vec{v}_1 \vec{S}_1 \times \vec{v}_1 \cdot \vec{v}_2 - \frac{15}{2} \hat{n} \cdot \vec{v}_2 \hat{n} \cdot \vec{v}_1 \hat{n} \times \vec{S}_1 \cdot \vec{v}_1 - \frac{1}{2} \vec{v}_1 \cdot \vec{v}_1 \hat{n} \times \vec{S}_1 \cdot \vec{v}_1 + \frac{3}{2} \vec{v}_1 \cdot \vec{v}_2 \hat{n} \times \vec{S}_1 \cdot \vec{v}_1 \right) \}$$

{DiagSet[3, 2, 69],

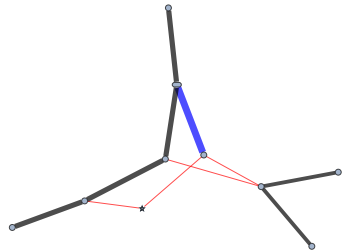

$$\frac{1}{r^3} G^3 m_1^2 m_2 \left( \frac{5}{4} \hat{n} \cdot \vec{a}_1 \hat{n} \times \vec{S}_1 \cdot \vec{v}_1 - \frac{1}{4} \hat{n} \cdot \vec{v}_1 \hat{n} \times \vec{a}_1 \cdot \vec{S}_1 - \frac{1}{2} \vec{a}_1 \times \vec{S}_1 \cdot \vec{v}_1 + \frac{3}{2} \hat{n} \cdot \vec{v}_1 \hat{n} \times \vec{S}_1 \cdot \vec{v}_1 \right) + \frac{1}{r^4} G^3 m_1^2 m_2 \left( -4 (\hat{n} \cdot \vec{v}_1)^2 \hat{n} \times \vec{S}_1 \cdot \vec{v}_1 - \frac{3}{2} \hat{n} \cdot \vec{v}_1 \vec{S}_1 \times \vec{v}_1 \cdot \vec{v}_2 + \frac{15}{2} \hat{n} \cdot \vec{v}_2 \hat{n} \cdot \vec{v}_1 \hat{n} \times \vec{S}_1 \cdot \vec{v}_1 + \vec{v}_1 \cdot \vec{v}_1 \hat{n} \times \vec{S}_1 \cdot \vec{v}_1 - \frac{3}{2} \vec{v}_1 \cdot \vec{v}_2 \hat{n} \times \vec{S}_1 \cdot \vec{v}_1 \right) \}$$

{DiagSet[3, 2, 70],

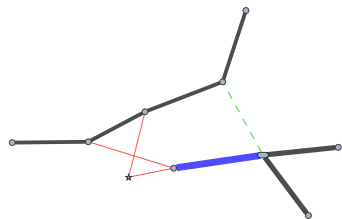

$$\frac{1}{r^3} G^3 m_2^3 \left( -\frac{2}{3} \hat{n} \cdot \vec{a}_2 \hat{n} \times \vec{S}_1 \cdot \vec{v}_2 + \frac{1}{3} \hat{n} \cdot \vec{v}_2 \hat{n} \times \vec{S}_1 \cdot \vec{a}_2 + \frac{2}{3} \vec{S}_1 \times \vec{v}_2 \cdot \vec{a}_2 - \frac{1}{3} \hat{n} \cdot \vec{v}_2 \hat{n} \times \vec{S}_1 \cdot \vec{v}_2 \right) + \frac{1}{r^4} G^3 m_2^3 \left( -\frac{7}{3} (\hat{n} \cdot \vec{v}_2)^2 \hat{n} \times \vec{S}_1 \cdot \vec{v}_2 + \frac{1}{3} \hat{n} \cdot \vec{v}_2 \vec{S}_1 \times \vec{v}_1 \cdot \vec{v}_2 + \frac{5}{3} \hat{n} \cdot \vec{v}_1 \hat{n} \cdot \vec{v}_2 \hat{n} \times \vec{S}_1 \cdot \vec{v}_2 - \frac{1}{3} \vec{v}_1 \cdot \vec{v}_2 \hat{n} \times \vec{S}_1 \cdot \vec{v}_2 - \frac{1}{3} \vec{v}_2 \cdot \vec{v}_2 \hat{n} \times \vec{S}_1 \cdot \vec{v}_2 \right) \}$$

{DiagSet[3, 2, 71],

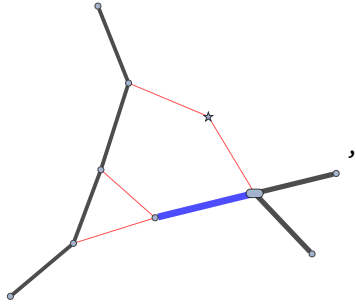

$$\frac{G^3 m_2^3 \left( \frac{1}{2} \hat{n} \cdot \vec{a}_1 \hat{n} \times \vec{S}_1 \cdot \vec{v}_2 + \frac{1}{2} \hat{n} \cdot \vec{v}_1 \hat{n} \times \vec{S}_1 \cdot \vec{v}_2 \right)}{r^3} + \frac{1}{r^4} G^3 m_2^3 \left( -\frac{5}{2} (\hat{n} \cdot \vec{v}_1)^2 \hat{n} \times \vec{S}_1 \cdot \vec{v}_2 - \frac{1}{2} \hat{n} \cdot \vec{v}_1 \vec{S}_1 \times \vec{v}_1 \cdot \vec{v}_2 + \right. \\ \left. \frac{3}{2} \hat{n} \cdot \vec{v}_2 \hat{n} \cdot \vec{v}_1 \hat{n} \times \vec{S}_1 \cdot \vec{v}_2 + \frac{1}{2} (\hat{n} \cdot \vec{v}_2)^2 \hat{n} \times \vec{S}_1 \cdot \vec{v}_1 + \frac{1}{2} \vec{v}_1 \cdot \vec{v}_1 \hat{n} \times \vec{S}_1 \cdot \vec{v}_2 - \frac{1}{2} \vec{v}_1 \cdot \vec{v}_2 \hat{n} \times \vec{S}_1 \cdot \vec{v}_2 - \frac{1}{2} \vec{v}_2 \cdot \vec{v}_2 \hat{n} \times \vec{S}_1 \cdot \vec{v}_1 \right) \Bigg\}$$

{DiagSet[3, 2, 72],

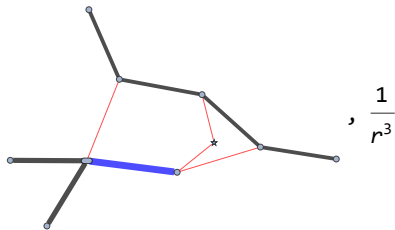

$$G^3 m_2^3 \left( -\frac{2}{3} \hat{n} \cdot \vec{a}_1 \hat{n} \times \vec{S}_1 \cdot \vec{v}_2 + \frac{1}{3} \hat{n} \cdot \vec{v}_2 \hat{n} \times \vec{S}_1 \cdot \vec{a}_1 + \frac{2}{3} \vec{S}_1 \times \vec{a}_1 \cdot \vec{v}_2 - \frac{2}{3} \hat{n} \cdot \vec{v}_1 \hat{n} \times \vec{S}_1 \cdot \vec{v}_2 + \frac{1}{3} \hat{n} \cdot \vec{v}_2 \hat{n} \times \vec{S}_1 \cdot \vec{v}_1 + \frac{2}{3} \vec{S}_1 \times \vec{v}_1 \cdot \vec{v}_2 \right) + \\ \frac{1}{r^4} G^3 m_2^3 \left( \frac{10}{3} (\hat{n} \cdot \vec{v}_1)^2 \hat{n} \times \vec{S}_1 \cdot \vec{v}_2 - \frac{4}{3} \hat{n} \cdot \vec{v}_1 \vec{S}_1 \times \vec{v}_1 \cdot \vec{v}_2 - \frac{5}{3} \hat{n} \cdot \vec{v}_2 \hat{n} \cdot \vec{v}_1 \hat{n} \times \vec{S}_1 \cdot \vec{v}_1 - 3 \hat{n} \cdot \vec{v}_2 \hat{n} \cdot \vec{v}_1 \hat{n} \times \vec{S}_1 \cdot \vec{v}_2 + \right. \\ \left. 2 (\hat{n} \cdot \vec{v}_2)^2 \hat{n} \times \vec{S}_1 \cdot \vec{v}_1 + 2 \hat{n} \cdot \vec{v}_2 \vec{S}_1 \times \vec{v}_1 \cdot \vec{v}_2 - \frac{2}{3} \vec{v}_1 \cdot \vec{v}_1 \hat{n} \times \vec{S}_1 \cdot \vec{v}_2 + \frac{1}{3} \vec{v}_1 \cdot \vec{v}_2 \hat{n} \times \vec{S}_1 \cdot \vec{v}_1 - \vec{v}_2 \cdot \vec{v}_2 \hat{n} \times \vec{S}_1 \cdot \vec{v}_1 \right) \Bigg\}$$

{DiagSet[3, 2, 73],

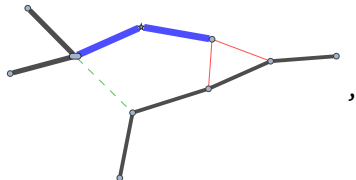

$$\frac{1}{r^3} G^3 m_2^3 \left( -\frac{1}{6} \hat{n} \cdot \vec{a}_2 \hat{n} \times \vec{S}_1 \cdot \vec{v}_2 - \frac{7}{6} \hat{n} \cdot \vec{v}_2 \hat{n} \times \vec{S}_1 \cdot \vec{a}_2 + \frac{1}{6} \vec{S}_1 \times \vec{v}_2 \cdot \vec{a}_2 - \frac{4}{3} \hat{n} \cdot \vec{v}_2 \hat{n} \times \vec{S}_1 \cdot \vec{v}_2 \right) + \frac{1}{r^4} \\ G^3 m_2^3 \left( -4 (\hat{n} \cdot \vec{v}_2)^2 \hat{n} \times \vec{S}_1 \cdot \vec{v}_2 + \frac{4}{3} \hat{n} \cdot \vec{v}_2 \vec{S}_1 \times \vec{v}_1 \cdot \vec{v}_2 + \frac{20}{3} \hat{n} \cdot \vec{v}_1 \hat{n} \cdot \vec{v}_2 \hat{n} \times \vec{S}_1 \cdot \vec{v}_2 - \frac{4}{3} \vec{v}_1 \cdot \vec{v}_2 \hat{n} \times \vec{S}_1 \cdot \vec{v}_2 \right) \Bigg\}$$

{DiagSet[3, 2, 74],

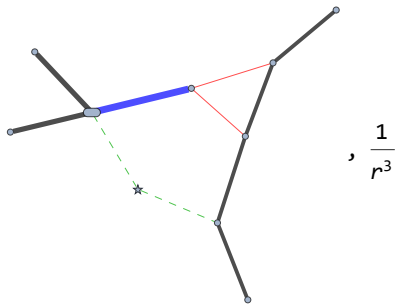

$$G^3 m_2^3 \left( -\frac{1}{2} \hat{n} \cdot \vec{a}_2 \hat{n} \times \vec{S}_1 \cdot \vec{v}_2 + \frac{3}{2} \hat{n} \cdot \vec{v}_1 \hat{n} \times \vec{S}_1 \cdot \vec{a}_2 - \frac{1}{2} \hat{n} \cdot \vec{v}_2 \hat{n} \times \vec{S}_1 \cdot \vec{a}_2 + \frac{1}{2} \vec{S}_1 \times \vec{v}_1 \cdot \vec{a}_2 + \frac{1}{2} \vec{S}_1 \times \vec{v}_2 \cdot \vec{a}_2 - \frac{1}{2} \hat{n} \cdot \vec{v}_2 \hat{n} \times \vec{S}_1 \cdot \vec{v}_2 \right) -$$

$$\frac{G^3 m_2^3 \hat{n} \times \vec{S}_1 \cdot \vec{a}_2}{2 r^2} + \frac{1}{r^4}$$

$$G^3 m_2^3 \left\{ (\hat{n} \cdot \vec{v}_2)^2 \left( -(\hat{n} \times \vec{S}_1 \cdot \vec{v}_2) \right) + \frac{1}{2} \hat{n} \cdot \vec{v}_2 \vec{S}_1 \times \vec{v}_1 \cdot \vec{v}_2 + \frac{5}{2} \hat{n} \cdot \vec{v}_1 \hat{n} \cdot \vec{v}_2 \hat{n} \times \vec{S}_1 \cdot \vec{v}_2 - \frac{1}{2} \vec{v}_1 \cdot \vec{v}_2 \hat{n} \times \vec{S}_1 \cdot \vec{v}_2 \right\}$$

{DiagSet[3, 2, 75], 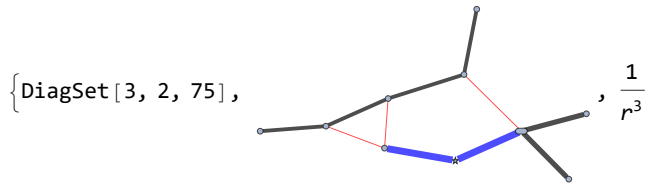 ,  $\frac{1}{r^3}$

$$G^3 m_2^3 \left( -\frac{1}{6} \hat{n} \cdot \vec{a}_1 \hat{n} \times \vec{S}_1 \cdot \vec{v}_2 - \frac{1}{6} \hat{n} \cdot \vec{v}_2 \hat{n} \times \vec{S}_1 \cdot \vec{a}_1 + \frac{1}{6} \vec{S}_1 \times \vec{a}_1 \cdot \vec{v}_2 - \frac{1}{6} \hat{n} \cdot \vec{v}_1 \hat{n} \times \vec{S}_1 \cdot \vec{v}_2 - \frac{1}{6} \hat{n} \cdot \vec{v}_2 \hat{n} \times \vec{S}_1 \cdot \vec{v}_1 + \frac{1}{6} \vec{S}_1 \times \vec{v}_1 \cdot \vec{v}_2 \right) +$$

$$\frac{1}{r^4} G^3 m_2^3 \left\{ \frac{5}{6} (\hat{n} \cdot \vec{v}_1)^2 \hat{n} \times \vec{S}_1 \cdot \vec{v}_2 - \frac{1}{3} \hat{n} \cdot \vec{v}_1 \vec{S}_1 \times \vec{v}_1 \cdot \vec{v}_2 + \frac{5}{6} \hat{n} \cdot \vec{v}_2 \hat{n} \cdot \vec{v}_1 \hat{n} \times \vec{S}_1 \cdot \vec{v}_1 - \right.$$

$$\frac{1}{6} \hat{n} \cdot \vec{v}_2 \hat{n} \cdot \vec{v}_1 \hat{n} \times \vec{S}_1 \cdot \vec{v}_2 - \frac{1}{6} (\hat{n} \cdot \vec{v}_2)^2 \hat{n} \times \vec{S}_1 \cdot \vec{v}_1 + \frac{1}{3} \hat{n} \cdot \vec{v}_2 \vec{S}_1 \times \vec{v}_1 \cdot \vec{v}_2 -$$

$$\left. \frac{1}{6} \vec{v}_1 \cdot \vec{v}_1 \hat{n} \times \vec{S}_1 \cdot \vec{v}_2 - \frac{1}{6} \vec{v}_1 \cdot \vec{v}_2 \hat{n} \times \vec{S}_1 \cdot \vec{v}_1 - \frac{1}{6} \vec{v}_1 \cdot \vec{v}_2 \hat{n} \times \vec{S}_1 \cdot \vec{v}_2 - \frac{1}{6} \vec{v}_2 \cdot \vec{v}_2 \hat{n} \times \vec{S}_1 \cdot \vec{v}_1 \right\}$$

{DiagSet[3, 2, 76], 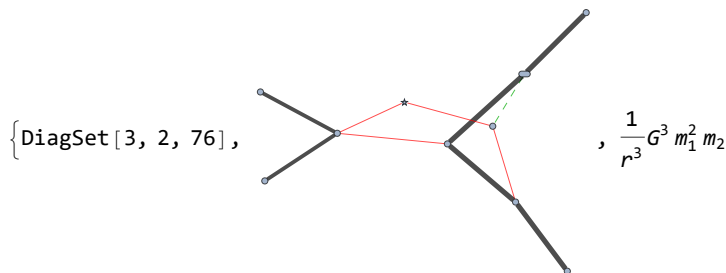 ,  $\frac{1}{r^3} G^3 m_1^2 m_2$

$$\left( -\frac{1}{4} \hat{n} \cdot \vec{v}_1 \hat{n} \times \vec{a}_1 \cdot \vec{S}_1 + \frac{3}{4} \hat{n} \cdot \vec{v}_2 \hat{n} \times \vec{a}_1 \cdot \vec{S}_1 - \frac{1}{4} \vec{a}_1 \times \vec{S}_1 \cdot \vec{v}_2 + \frac{1}{4} \hat{n} \cdot \vec{v}_1 \hat{n} \times \vec{S}_1 \cdot \vec{v}_1 - \frac{3}{4} \hat{n} \cdot \vec{v}_2 \hat{n} \times \vec{S}_1 \cdot \vec{v}_1 + \frac{1}{4} \vec{S}_1 \times \vec{v}_1 \cdot \vec{v}_2 \right) +$$

$$\frac{1}{r^4} G^3 m_1^2 m_2 \left\{ -\frac{1}{2} (\hat{n} \cdot \vec{v}_1)^2 \hat{n} \times \vec{S}_1 \cdot \vec{v}_1 - \frac{1}{2} \hat{n} \cdot \vec{v}_1 \vec{S}_1 \times \vec{v}_1 \cdot \vec{v}_2 + \frac{5}{2} \hat{n} \cdot \vec{v}_2 \hat{n} \cdot \vec{v}_1 \hat{n} \times \vec{S}_1 \cdot \vec{v}_1 - \frac{1}{2} \vec{v}_1 \cdot \vec{v}_2 \hat{n} \times \vec{S}_1 \cdot \vec{v}_1 \right\}$$

{DiagSet[3, 2, 77], 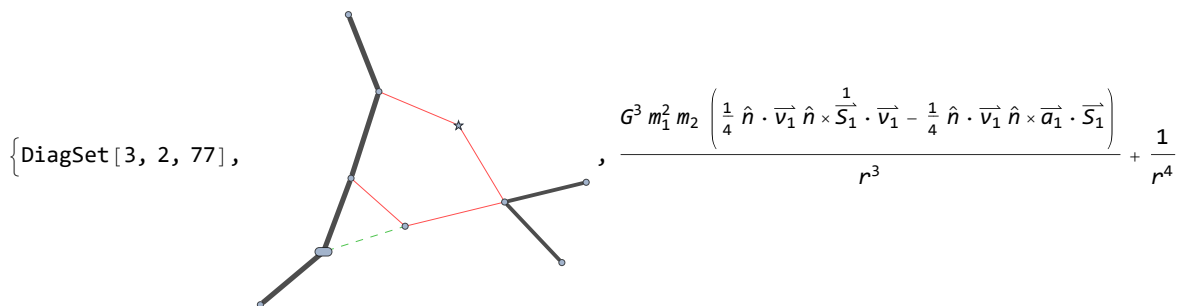 ,  $\frac{G^3 m_1^2 m_2 \left( \frac{1}{4} \hat{n} \cdot \vec{v}_1 \hat{n} \times \vec{S}_1 \cdot \vec{v}_1 - \frac{1}{4} \hat{n} \cdot \vec{v}_1 \hat{n} \times \vec{a}_1 \cdot \vec{S}_1 \right)}{r^3} + \frac{1}{r^4}$

$$G^3 m_1^2 m_2 \left\{ (\hat{n} \cdot \vec{v}_1)^2 \left( -(\hat{n} \times \vec{S}_1 \cdot \vec{v}_1) \right) - \frac{1}{4} \hat{n} \cdot \vec{v}_1 \vec{S}_1 \times \vec{v}_1 \cdot \vec{v}_2 + \frac{5}{4} \hat{n} \cdot \vec{v}_2 \hat{n} \cdot \vec{v}_1 \hat{n} \times \vec{S}_1 \cdot \vec{v}_1 - \frac{1}{4} \vec{v}_1 \cdot \vec{v}_2 \hat{n} \times \vec{S}_1 \cdot \vec{v}_1 \right\}$$

{DiagSet[3, 2, 78], 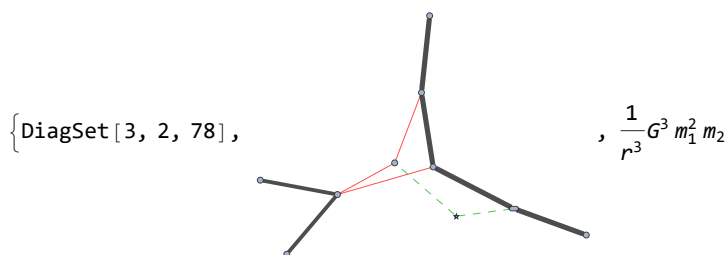 ,  $\frac{1}{r^3} G^3 m_1^2 m_2$

$$\left( \frac{1}{4} \hat{n} \cdot \vec{a}_1 \hat{n} \times \vec{S}_1 \cdot \vec{v}_1 + \frac{3}{2} \hat{n} \cdot \vec{a}_2 \hat{n} \times \vec{S}_1 \cdot \vec{v}_1 + \frac{1}{4} \hat{n} \cdot \vec{v}_1 \hat{n} \times \vec{a}_1 \cdot \vec{S}_1 - \frac{1}{2} \vec{a}_1 \times \vec{S}_1 \cdot \vec{v}_1 - \frac{1}{2} \vec{a}_2 \times \vec{S}_1 \cdot \vec{v}_1 - \frac{3}{2} \hat{n} \cdot \vec{v}_1 \hat{n} \times \vec{S}_1 \cdot \vec{v}_1 \right) -$$

$$\frac{G^3 m_1^2 m_2 \hat{n} \times \vec{a}_1 \cdot \vec{S}_1}{2 r^2} + \frac{1}{r^4} G^3 m_1^2 m_2 \left( \frac{15}{2} (\hat{n} \cdot \vec{v}_2)^2 \hat{n} \times \vec{S}_1 \cdot \vec{v}_1 - 3 \hat{n} \cdot \vec{v}_2 \vec{S}_1 \times \vec{v}_1 \cdot \vec{v}_2 - 5 \hat{n} \cdot \vec{v}_1 \hat{n} \cdot \vec{v}_2 \hat{n} \times \vec{S}_1 \cdot \vec{v}_1 + \right.$$

$$\left. \hat{n} \cdot \vec{v}_1 \vec{S}_1 \times \vec{v}_1 \cdot \vec{v}_2 - \frac{1}{2} \vec{v}_1 \cdot \vec{v}_1 \hat{n} \times \vec{S}_1 \cdot \vec{v}_1 + \vec{v}_1 \cdot \vec{v}_2 \hat{n} \times \vec{S}_1 \cdot \vec{v}_1 - \frac{3}{2} \vec{v}_2 \cdot \vec{v}_2 \hat{n} \times \vec{S}_1 \cdot \vec{v}_1 \right) \Bigg\}$$

{DiagSet[3, 2, 79],

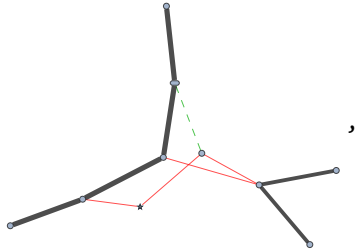

$$\frac{1}{r^3} G^3 m_1^2 m_2 \left( \frac{3}{4} \hat{n} \cdot \vec{a}_1 \hat{n} \times \vec{S}_1 \cdot \vec{v}_1 - \frac{3}{2} \hat{n} \cdot \vec{a}_2 \hat{n} \times \vec{S}_1 \cdot \vec{v}_1 + \frac{5}{4} \hat{n} \cdot \vec{v}_1 \hat{n} \times \vec{a}_1 \cdot \vec{S}_1 - \frac{3}{2} \hat{n} \cdot \vec{v}_2 \hat{n} \times \vec{a}_1 \cdot \vec{S}_1 - \right.$$

$$\left. \frac{1}{2} \vec{a}_1 \times \vec{S}_1 \cdot \vec{v}_1 + \frac{1}{2} \vec{a}_1 \times \vec{S}_1 \cdot \vec{v}_2 + \frac{1}{2} \vec{a}_2 \times \vec{S}_1 \cdot \vec{v}_1 - \frac{3}{2} \hat{n} \cdot \vec{v}_2 \hat{n} \times \vec{S}_1 \cdot \vec{v}_1 + \frac{1}{2} \vec{S}_1 \times \vec{v}_1 \cdot \vec{v}_2 \right) -$$

$$\frac{G^3 m_1^2 m_2 \hat{n} \times \vec{a}_1 \cdot \vec{S}_1}{2 r^2} + \frac{1}{r^4} G^3 m_1^2 m_2 \left( (\hat{n} \cdot \vec{v}_1)^2 \left( -(\hat{n} \times \vec{S}_1 \cdot \vec{v}_1) \right) - \hat{n} \cdot \vec{v}_1 \vec{S}_1 \times \vec{v}_1 \cdot \vec{v}_2 + 5 \hat{n} \cdot \vec{v}_2 \hat{n} \cdot \vec{v}_1 \hat{n} \times \vec{S}_1 \cdot \vec{v}_1 - \right.$$

$$\left. \frac{15}{2} (\hat{n} \cdot \vec{v}_2)^2 \hat{n} \times \vec{S}_1 \cdot \vec{v}_1 + 3 \hat{n} \cdot \vec{v}_2 \vec{S}_1 \times \vec{v}_1 \cdot \vec{v}_2 - \vec{v}_1 \cdot \vec{v}_2 \hat{n} \times \vec{S}_1 \cdot \vec{v}_1 + \frac{3}{2} \vec{v}_2 \cdot \vec{v}_2 \hat{n} \times \vec{S}_1 \cdot \vec{v}_1 \right) \Bigg\}$$

{DiagSet[3, 2, 80],

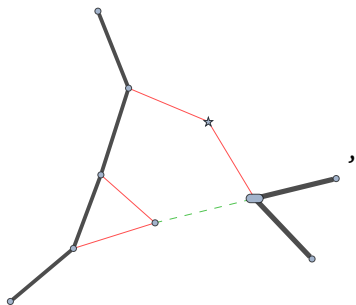

$$, \frac{G^3 m_2^3 \left( \hat{n} \cdot \vec{v}_2 \left( -\left( \hat{n} \times \vec{S}_1 \cdot \vec{v}_2 \right) \right) - \hat{n} \cdot \vec{v}_2 \hat{n} \times \vec{S}_1 \cdot \vec{a}_2 \right)}{r^3} +$$

$$\frac{1}{r^4} G^3 m_2^3 \left( -4 (\hat{n} \cdot \vec{v}_2)^2 \hat{n} \times \vec{S}_1 \cdot \vec{v}_2 + \hat{n} \cdot \vec{v}_2 \vec{S}_1 \times \vec{v}_1 \cdot \vec{v}_2 + 5 \hat{n} \cdot \vec{v}_1 \hat{n} \cdot \vec{v}_2 \hat{n} \times \vec{S}_1 \cdot \vec{v}_2 - \vec{v}_1 \cdot \vec{v}_2 \hat{n} \times \vec{S}_1 \cdot \vec{v}_2 \right) \Bigg\}$$

{DiagSet[3, 2, 81],

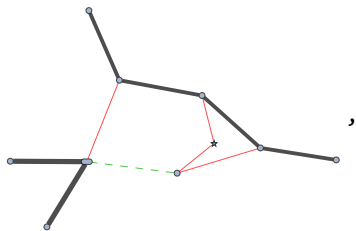

$$\frac{1}{r^3} G^3 m_2^3 \left( -4 \hat{n} \cdot \vec{a}_2 \hat{n} \times \vec{S}_1 \cdot \vec{v}_2 - 6 \hat{n} \cdot \vec{v}_1 \hat{n} \times \vec{S}_1 \cdot \vec{a}_2 + 6 \hat{n} \cdot \vec{v}_2 \hat{n} \times \vec{S}_1 \cdot \vec{a}_2 - 2 \vec{S}_1 \times \vec{v}_1 \cdot \vec{a}_2 + 4 \vec{S}_1 \times \vec{v}_2 \cdot \vec{a}_2 \right) +$$

$$\frac{2 G^3 m_2^3 \hat{n} \times \vec{S}_1 \cdot \vec{a}_2}{r^2} + \frac{G^3 m_2^3 \left( -4 (\hat{n} \cdot \vec{v}_2)^2 \hat{n} \times \vec{S}_1 \cdot \vec{v}_2 - 2 \vec{v}_2 \cdot \vec{v}_2 \hat{n} \times \vec{S}_1 \cdot \vec{v}_2 \right)}{r^4} \Bigg\}$$

{DiagSet[3, 2, 82],

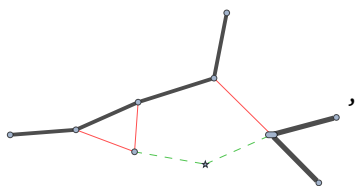

$$\frac{G^3 m_2^3 \left( 3 \hat{n} \cdot \vec{v}_1 \hat{n} \times \vec{S}_1 \cdot \vec{a}_2 - \hat{n} \cdot \vec{v}_2 \hat{n} \times \vec{S}_1 \cdot \vec{a}_2 + \vec{S}_1 \times \vec{v}_1 \cdot \vec{a}_2 - 2 \hat{n} \cdot \vec{v}_2 \hat{n} \times \vec{S}_1 \cdot \vec{v}_2 \right)}{r^3} - \frac{G^3 m_2^3 \hat{n} \times \vec{S}_1 \cdot \vec{a}_2}{r^2} + \frac{1}{r^4}$$

$$G^3 m_2^3 \left( -2 (\hat{n} \cdot \vec{v}_2)^2 \hat{n} \times \vec{S}_1 \cdot \vec{v}_2 + 2 \hat{n} \cdot \vec{v}_2 \vec{S}_1 \times \vec{v}_1 \cdot \vec{v}_2 + 10 \hat{n} \cdot \vec{v}_1 \hat{n} \cdot \vec{v}_2 \hat{n} \times \vec{S}_1 \cdot \vec{v}_2 - 2 \vec{v}_1 \cdot \vec{v}_2 \hat{n} \times \vec{S}_1 \cdot \vec{v}_2 \right) \}$$

{DiagSet[3, 3, 1],

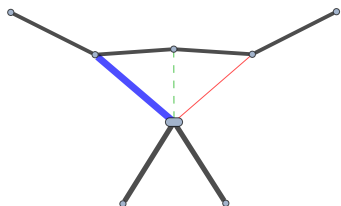

$$, \frac{16 G^3 m_2^3 \vec{v}_2 \cdot \vec{v}_2 \hat{n} \times \vec{S}_1 \cdot \vec{v}_2}{r^4} \}$$

{DiagSet[3, 3, 2],

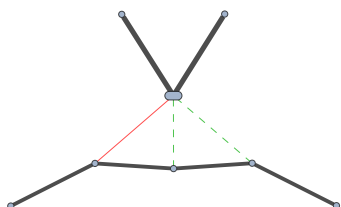

$$, \frac{32 G^3 m_2^3 \vec{v}_1 \cdot \vec{v}_2 \hat{n} \times \vec{S}_1 \cdot \vec{v}_2}{r^4} - \frac{32 G^3 m_2^3 \vec{S}_1 \times \vec{v}_2 \cdot \vec{a}_2}{r^3} \}$$

{DiagSet[3, 3, 3],

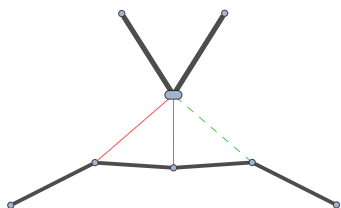

$$, - \frac{56 G^3 m_2^3 \vec{v}_2 \cdot \vec{v}_2 \hat{n} \times \vec{S}_1 \cdot \vec{v}_2}{r^4} \}$$

{DiagSet[3, 3, 4],

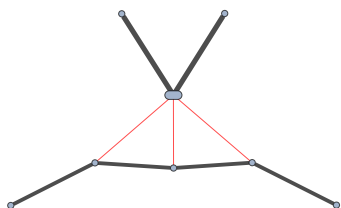

$$, \frac{16 G^3 m_2^3 \vec{S}_1 \times \vec{v}_1 \cdot \vec{a}_1}{3 r^3} + \frac{8 G^3 m_2^3 \vec{v}_1 \cdot \vec{v}_1 \hat{n} \times \vec{S}_1 \cdot \vec{v}_1}{r^4} \}$$

{DiagSet[3, 3, 5],

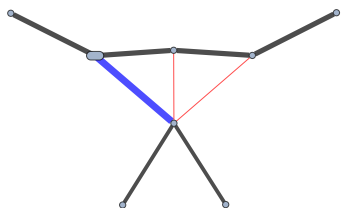

$$, \frac{G^3 m_1^2 m_2 \left( 9 \vec{v}_1 \cdot \vec{v}_2 \hat{n} \times \vec{S}_1 \cdot \vec{v}_2 - 9 \vec{v}_2 \cdot \vec{v}_2 \hat{n} \times \vec{S}_1 \cdot \vec{v}_1 \right)}{r^4} \}$$

{DiagSet[3, 3, 6],

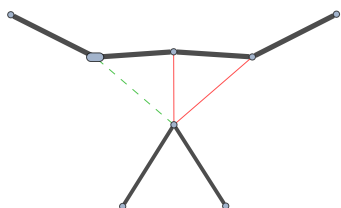

$$, \frac{G^3 m_1^2 m_2 \left( 2 \vec{S}_1 \times \vec{v}_1 \cdot \vec{v}_2 - 2 \vec{a}_1 \times \vec{S}_1 \cdot \vec{v}_2 \right)}{r^3} +$$

$$\frac{1}{r^4} G^3 m_1^2 m_2 \left( -\frac{1}{2} \hat{n} \cdot \vec{v}_1 \vec{S}_1 \times \vec{v}_1 \cdot \vec{v}_2 - 3 \vec{v}_1 \cdot \vec{v}_1 \hat{n} \times \vec{S}_1 \cdot \vec{v}_2 - \frac{3}{2} \vec{v}_1 \cdot \vec{v}_2 \hat{n} \times \vec{S}_1 \cdot \vec{v}_1 - \frac{9}{2} \vec{v}_2 \cdot \vec{v}_2 \hat{n} \times \vec{S}_1 \cdot \vec{v}_2 \right) \Bigg\}$$

$$\left\{ \text{DiagSet}[3, 3, 7], \right. \quad \left. -\frac{8 G^3 m_1^2 m_2 \vec{v}_1 \cdot \vec{v}_2 \hat{n} \times \vec{S}_1 \cdot \vec{v}_1}{r^4} \right\}$$
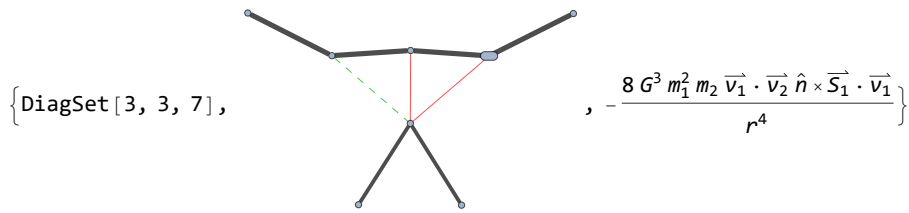

$$\left\{ \text{DiagSet}[3, 3, 8], \right. \quad \left. , \right.$$
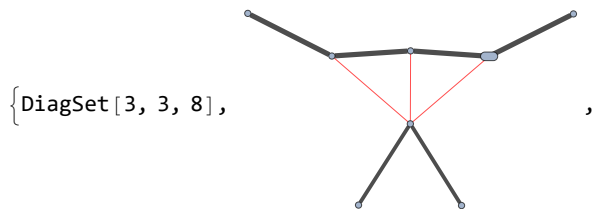

$$\frac{G^3 m_1^2 m_2 \vec{a}_1 \times \vec{S}_1 \cdot \vec{v}_1}{r^3} + \frac{G^3 m_1^2 m_2 \left( \frac{7}{2} \vec{v}_1 \cdot \vec{v}_1 \hat{n} \times \vec{S}_1 \cdot \vec{v}_1 + \frac{27}{2} \vec{v}_2 \cdot \vec{v}_2 \hat{n} \times \vec{S}_1 \cdot \vec{v}_1 \right)}{r^4} \Bigg\}$$

$$\left\{ \text{DiagSet}[3, 3, 9], \right. \quad \left. , \right.$$
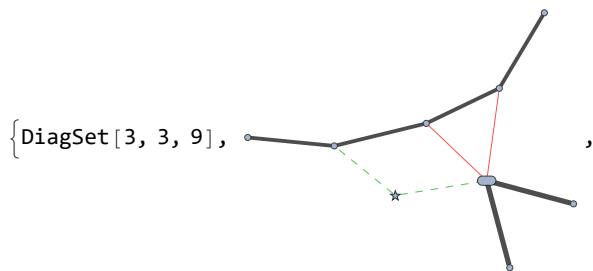

$$\frac{G^3 m_2^3 \left( 24 \hat{n} \cdot \vec{v}_1 \hat{n} \times \vec{S}_1 \cdot \vec{a}_2 - 16 \hat{n} \cdot \vec{v}_2 \hat{n} \times \vec{S}_1 \cdot \vec{a}_2 + 8 \vec{S}_1 \times \vec{v}_1 \cdot \vec{a}_2 - 8 \hat{n} \cdot \vec{v}_2 \hat{n} \times \vec{S}_1 \cdot \vec{v}_2 \right)}{r^3} - \frac{8 G^3 m_2^3 \hat{n} \times \vec{S}_1 \cdot \vec{a}_2}{r^2} +$$

$$\frac{1}{r^4} G^3 m_2^3 \left( -16 (\hat{n} \cdot \vec{v}_2)^2 \hat{n} \times \vec{S}_1 \cdot \vec{v}_2 + 8 \hat{n} \cdot \vec{v}_2 \vec{S}_1 \times \vec{v}_1 \cdot \vec{v}_2 + 40 \hat{n} \cdot \vec{v}_1 \hat{n} \cdot \vec{v}_2 \hat{n} \times \vec{S}_1 \cdot \vec{v}_2 - 8 \vec{v}_1 \cdot \vec{v}_2 \hat{n} \times \vec{S}_1 \cdot \vec{v}_2 \right) \Bigg\}$$

$$\left\{ \text{DiagSet}[3, 3, 10], \right. \quad \left. , \right.$$
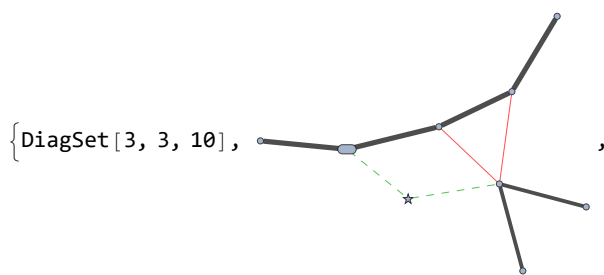

$$\frac{1}{r^3} G^3 m_1^2 m_2 \left( -\frac{1}{2} \hat{n} \cdot \vec{v}_1 \hat{n} \times \vec{a}_2 \cdot \vec{S}_1 + \frac{1}{2} \vec{a}_2 \times \vec{S}_1 \cdot \vec{v}_1 + \hat{n} \cdot \vec{v}_1 \hat{n} \times \vec{S}_1 \cdot \vec{v}_2 - \frac{3}{2} \hat{n} \cdot \vec{v}_2 \hat{n} \times \vec{S}_1 \cdot \vec{v}_2 \right) + \frac{G^3 m_1^2 m_2 \hat{n} \times \vec{a}_2 \cdot \vec{S}_1}{2 r^2} + \frac{1}{r^4} G^3 m_1^2 m_2$$

$$\left( (\hat{n} \cdot \vec{v}_1)^2 \left( -(\hat{n} \times \vec{S}_1 \cdot \vec{v}_2) \right) - \hat{n} \cdot \vec{v}_1 \vec{S}_1 \times \vec{v}_1 \cdot \vec{v}_2 + \frac{5}{2} \hat{n} \cdot \vec{v}_2 \hat{n} \cdot \vec{v}_1 \hat{n} \times \vec{S}_1 \cdot \vec{v}_2 + \frac{3}{2} \hat{n} \cdot \vec{v}_2 \vec{S}_1 \times \vec{v}_1 \cdot \vec{v}_2 - \frac{1}{2} \vec{v}_1 \cdot \vec{v}_2 \hat{n} \times \vec{S}_1 \cdot \vec{v}_2 \right) \Bigg\}$$

$$\left\{ \text{DiagSet}[3, 3, 11], \right. , \frac{G^3 m_1^2 m_2 \left( \hat{n} \cdot \vec{v}_1 \hat{n} \times \vec{a}_1 \cdot \vec{S}_1 - \hat{n} \cdot \vec{v}_1 \hat{n} \times \vec{S}_1 \cdot \vec{v}_1 \right)}{r^3} +$$
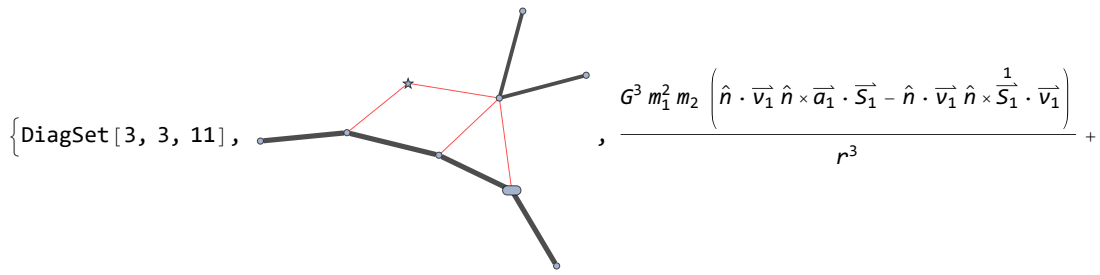

$$\frac{1}{r^4} G^3 m_1^2 m_2 \left( 4 \left( \hat{n} \cdot \vec{v}_1 \right)^2 \hat{n} \times \vec{S}_1 \cdot \vec{v}_1 + \hat{n} \cdot \vec{v}_1 \vec{S}_1 \times \vec{v}_1 \cdot \vec{v}_2 - 5 \hat{n} \cdot \vec{v}_2 \hat{n} \cdot \vec{v}_1 \hat{n} \times \vec{S}_1 \cdot \vec{v}_1 + \vec{v}_1 \cdot \vec{v}_2 \hat{n} \times \vec{S}_1 \cdot \vec{v}_1 \right) \}$$

$$\left\{ \text{DiagSet}[3, 3, 12], \right. , \frac{G^3 m_2^3 \left( -16 \hat{n} \cdot \vec{v}_2 \hat{n} \times \vec{S}_1 \cdot \vec{a}_2 - 16 \hat{n} \cdot \vec{v}_2 \hat{n} \times \vec{S}_1 \cdot \vec{v}_2 \right)}{r^3} +$$
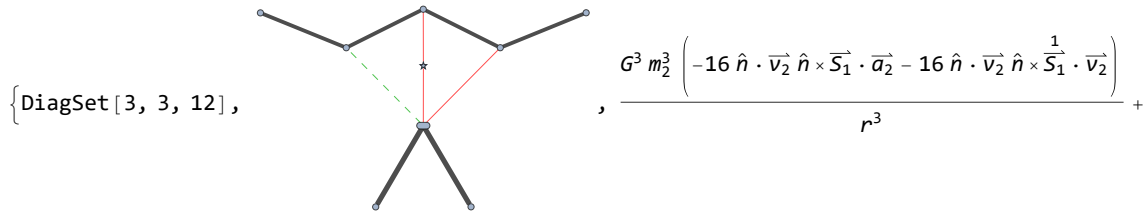

$$\frac{1}{r^4} G^3 m_2^3 \left( -64 \left( \hat{n} \cdot \vec{v}_2 \right)^2 \hat{n} \times \vec{S}_1 \cdot \vec{v}_2 + 16 \hat{n} \cdot \vec{v}_2 \vec{S}_1 \times \vec{v}_1 \cdot \vec{v}_2 + 80 \hat{n} \cdot \vec{v}_1 \hat{n} \cdot \vec{v}_2 \hat{n} \times \vec{S}_1 \cdot \vec{v}_2 - 16 \vec{v}_1 \cdot \vec{v}_2 \hat{n} \times \vec{S}_1 \cdot \vec{v}_2 \right) \}$$

$$\left\{ \text{DiagSet}[3, 3, 13], \right. , \frac{G^3 m_1^2 m_2 \left( \hat{n} \cdot \vec{v}_1 \hat{n} \times \vec{S}_1 \cdot \vec{v}_2 - \hat{n} \cdot \vec{v}_1 \hat{n} \times \vec{a}_2 \cdot \vec{S}_1 \right)}{r^3} +$$
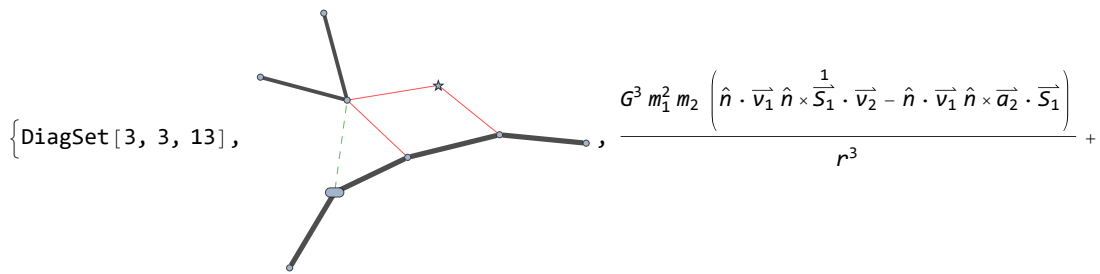

$$\frac{1}{r^4} G^3 m_1^2 m_2 \left( -4 \left( \hat{n} \cdot \vec{v}_1 \right)^2 \hat{n} \times \vec{S}_1 \cdot \vec{v}_2 - \hat{n} \cdot \vec{v}_1 \vec{S}_1 \times \vec{v}_1 \cdot \vec{v}_2 + 5 \hat{n} \cdot \vec{v}_2 \hat{n} \cdot \vec{v}_1 \hat{n} \times \vec{S}_1 \cdot \vec{v}_2 - \vec{v}_1 \cdot \vec{v}_2 \hat{n} \times \vec{S}_1 \cdot \vec{v}_2 \right) \}$$

$$\left\{ \text{DiagSet}[3, 3, 14], \right. ,$$
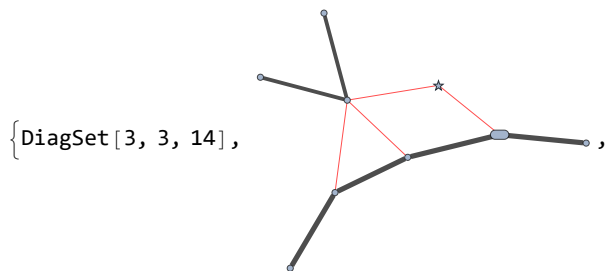

$$\frac{1}{r^3} G^3 m_1^2 m_2 \left( \hat{n} \cdot \vec{v}_1 \hat{n} \times \vec{a}_1 \cdot \vec{S}_1 - \frac{3}{2} \hat{n} \cdot \vec{v}_2 \hat{n} \times \vec{a}_1 \cdot \vec{S}_1 + \frac{1}{2} \vec{a}_1 \times \vec{S}_1 \cdot \vec{v}_2 - \hat{n} \cdot \vec{v}_1 \hat{n} \times \vec{S}_1 \cdot \vec{v}_1 + \frac{3}{2} \hat{n} \cdot \vec{v}_2 \hat{n} \times \vec{S}_1 \cdot \vec{v}_1 - \frac{1}{2} \vec{S}_1 \times \vec{v}_1 \cdot \vec{v}_2 \right) +$$

$$\frac{1}{r^4} G^3 m_1^2 m_2 \left( \left( \hat{n} \cdot \vec{v}_1 \right)^2 \hat{n} \times \vec{S}_1 \cdot \vec{v}_1 + \frac{1}{2} \hat{n} \cdot \vec{v}_1 \vec{S}_1 \times \vec{v}_1 \cdot \vec{v}_2 - \frac{5}{2} \hat{n} \cdot \vec{v}_2 \hat{n} \cdot \vec{v}_1 \hat{n} \times \vec{S}_1 \cdot \vec{v}_1 + \frac{1}{2} \vec{v}_1 \cdot \vec{v}_2 \hat{n} \times \vec{S}_1 \cdot \vec{v}_1 \right) \}$$

$$\left\{ \text{DiagSet}[3, 4, 1], \right. , \frac{G^3 m_1 m_2^2 \left( 6 \vec{v}_2 \cdot \vec{v}_2 \hat{n} \times \vec{S}_1 \cdot \vec{v}_1 - 6 \vec{v}_1 \cdot \vec{v}_2 \hat{n} \times \vec{S}_1 \cdot \vec{v}_2 \right)}{r^4} \}$$
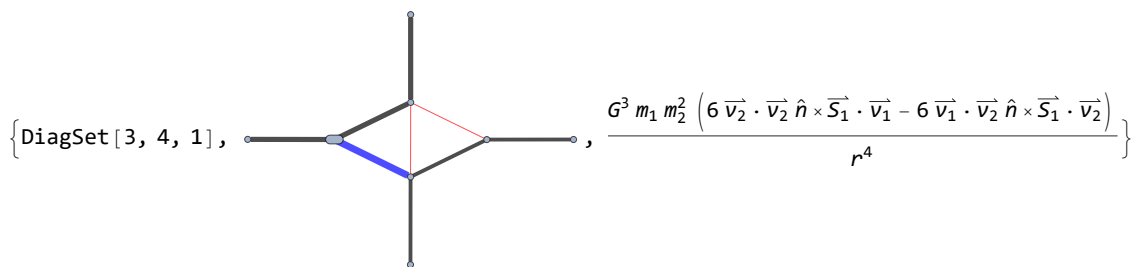

$$\left\{ \text{DiagSet}[3, 4, 2], \text{Diagram} \right\},$$

$$\frac{G^3 m_1 m_2^2 \left( 4 \vec{S}_1 \times \vec{a}_1 \cdot \vec{v}_2 + 4 \vec{S}_1 \times \vec{v}_1 \cdot \vec{v}_2 \right)}{r^3} + \frac{G^3 m_1 m_2^2 \left( \hat{n} \cdot \vec{v}_1 \left( - \left( \vec{S}_1 \times \vec{v}_1 \cdot \vec{v}_2 \right) \right) + 9 \vec{v}_1 \cdot \vec{v}_1 \hat{n} \times \vec{S}_1 \cdot \vec{v}_2 - 3 \vec{v}_1 \cdot \vec{v}_2 \hat{n} \times \vec{S}_1 \cdot \vec{v}_1 \right)}{r^4} \}$$

$$\left\{ \text{DiagSet}[3, 4, 3], \text{Diagram}, \frac{8 G^3 m_1 m_2^2 \vec{v}_1 \cdot \vec{v}_2 \hat{n} \times \vec{S}_1 \cdot \vec{v}_2}{r^4} \right\}$$

$$\left\{ \text{DiagSet}[3, 4, 4], \text{Diagram} \right\},$$

$$\frac{2 G^3 m_1 m_2^2 \vec{S}_1 \times \vec{v}_1 \cdot \vec{a}_1}{r^3} + \frac{G^3 m_1 m_2^2 \left( -8 \vec{v}_1 \cdot \vec{v}_1 \hat{n} \times \vec{S}_1 \cdot \vec{v}_1 - 6 \vec{v}_2 \cdot \vec{v}_2 \hat{n} \times \vec{S}_1 \cdot \vec{v}_1 \right)}{r^4} \}$$

$$\left\{ \text{DiagSet}[3, 4, 5], \text{Diagram}, -\frac{8 G^3 m_1 m_2^2 \vec{v}_1 \cdot \vec{v}_2 \hat{n} \times \vec{S}_1 \cdot \vec{v}_1}{r^4} \right\}$$

$$\left\{ \text{DiagSet}[3, 4, 6], \text{Diagram}, -\frac{8 G^3 m_1 m_2^2 \vec{v}_1 \cdot \vec{v}_2 \hat{n} \times \vec{S}_1 \cdot \vec{v}_1}{r^4} \right\}$$



|                               |                                                                                     |                                                                                                                                                                                               |
|-------------------------------|-------------------------------------------------------------------------------------|-----------------------------------------------------------------------------------------------------------------------------------------------------------------------------------------------|
| $\{\text{DiagSet}[3, 4, 7],$  | 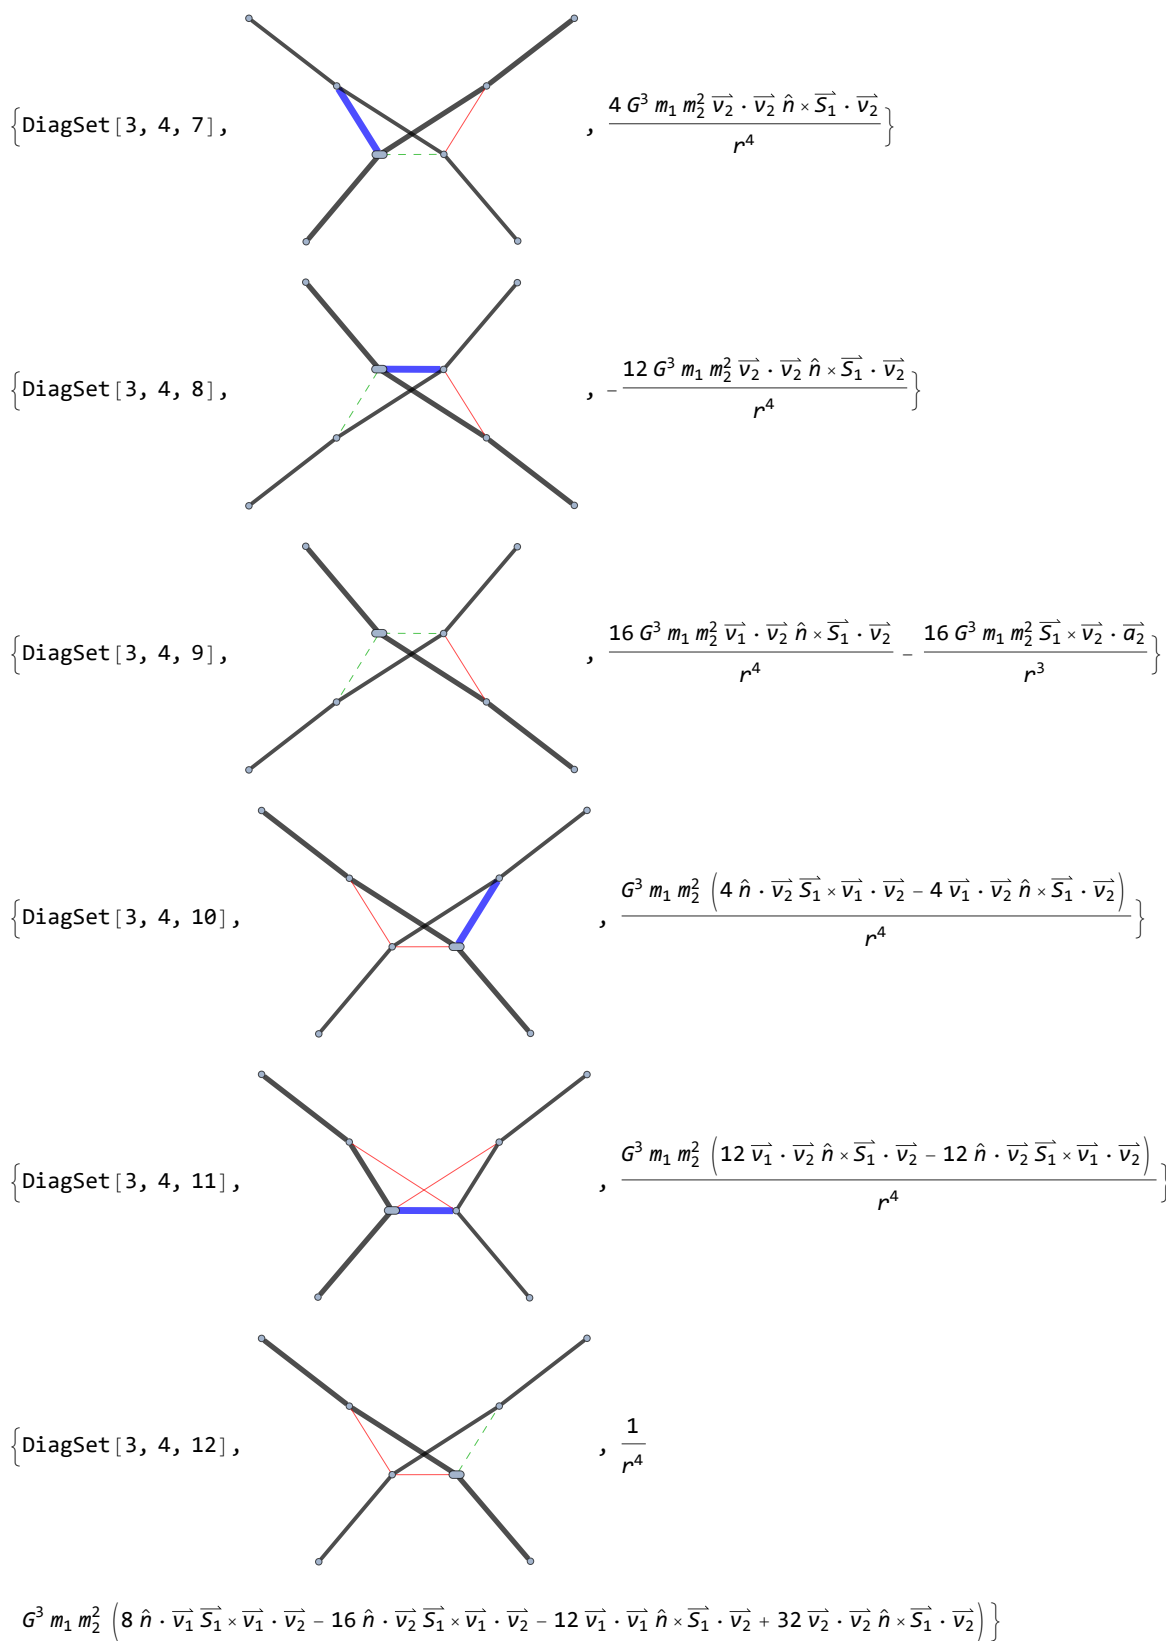   | $, \frac{4 G^3 m_1 m_2^2 \vec{v}_2 \cdot \vec{v}_2 \hat{n} \times \vec{S}_1 \cdot \vec{v}_2}{r^4} \}$                                                                                         |
| $\{\text{DiagSet}[3, 4, 8],$  | 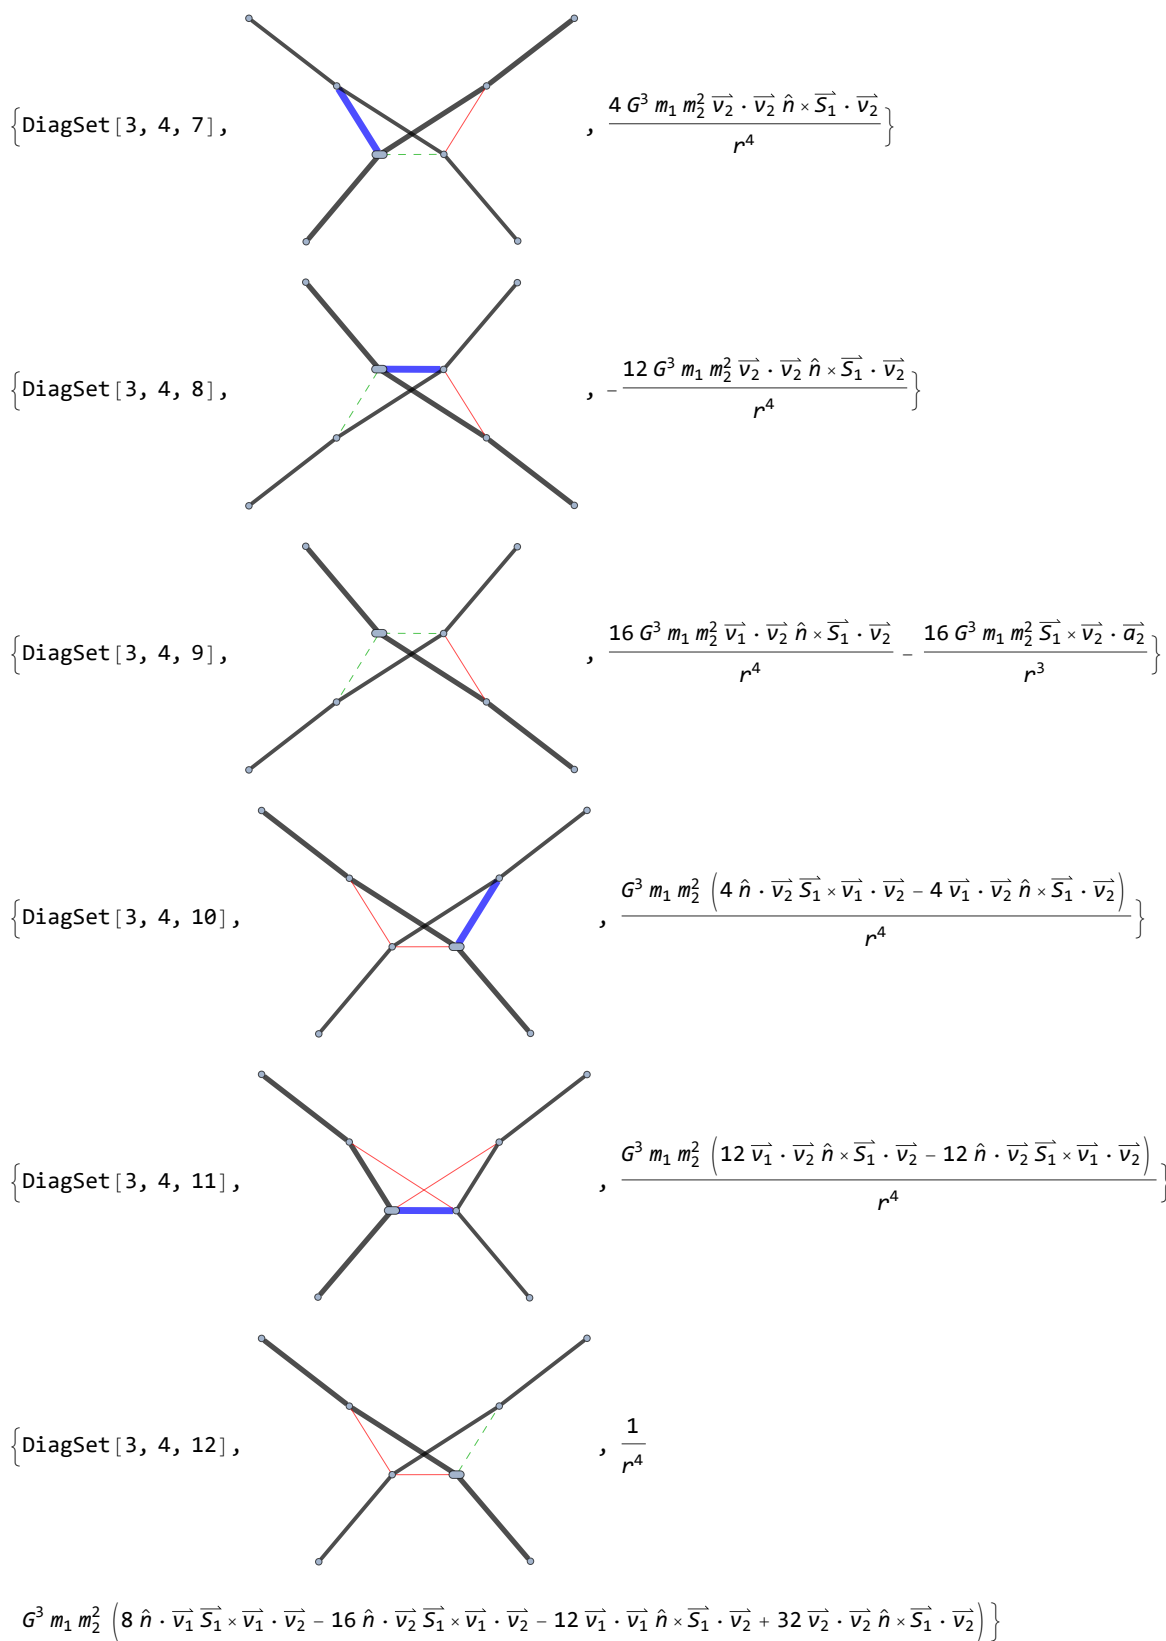   | $, - \frac{12 G^3 m_1 m_2^2 \vec{v}_2 \cdot \vec{v}_2 \hat{n} \times \vec{S}_1 \cdot \vec{v}_2}{r^4} \}$                                                                                      |
| $\{\text{DiagSet}[3, 4, 9],$  | 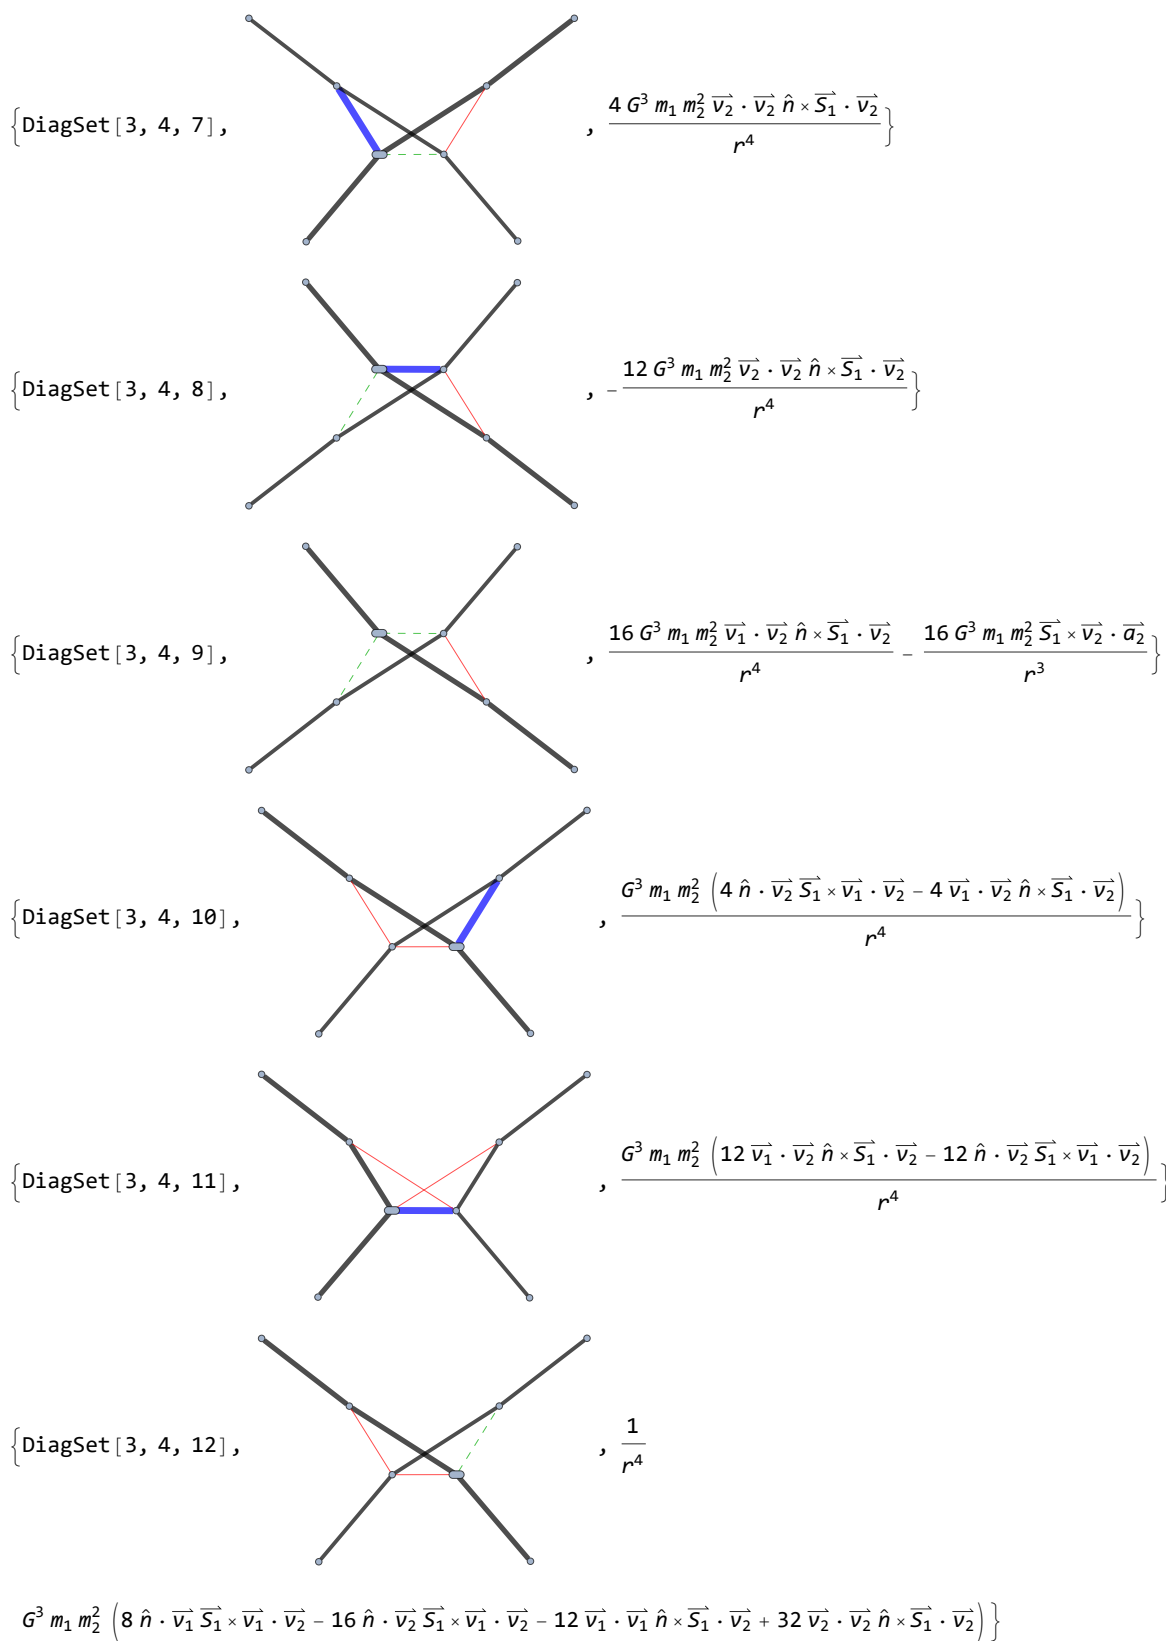   | $, \frac{16 G^3 m_1 m_2^2 \vec{v}_1 \cdot \vec{v}_2 \hat{n} \times \vec{S}_1 \cdot \vec{v}_2}{r^4} - \frac{16 G^3 m_1 m_2^2 \vec{S}_1 \times \vec{v}_2 \cdot \vec{a}_2}{r^3} \}$              |
| $\{\text{DiagSet}[3, 4, 10],$ | 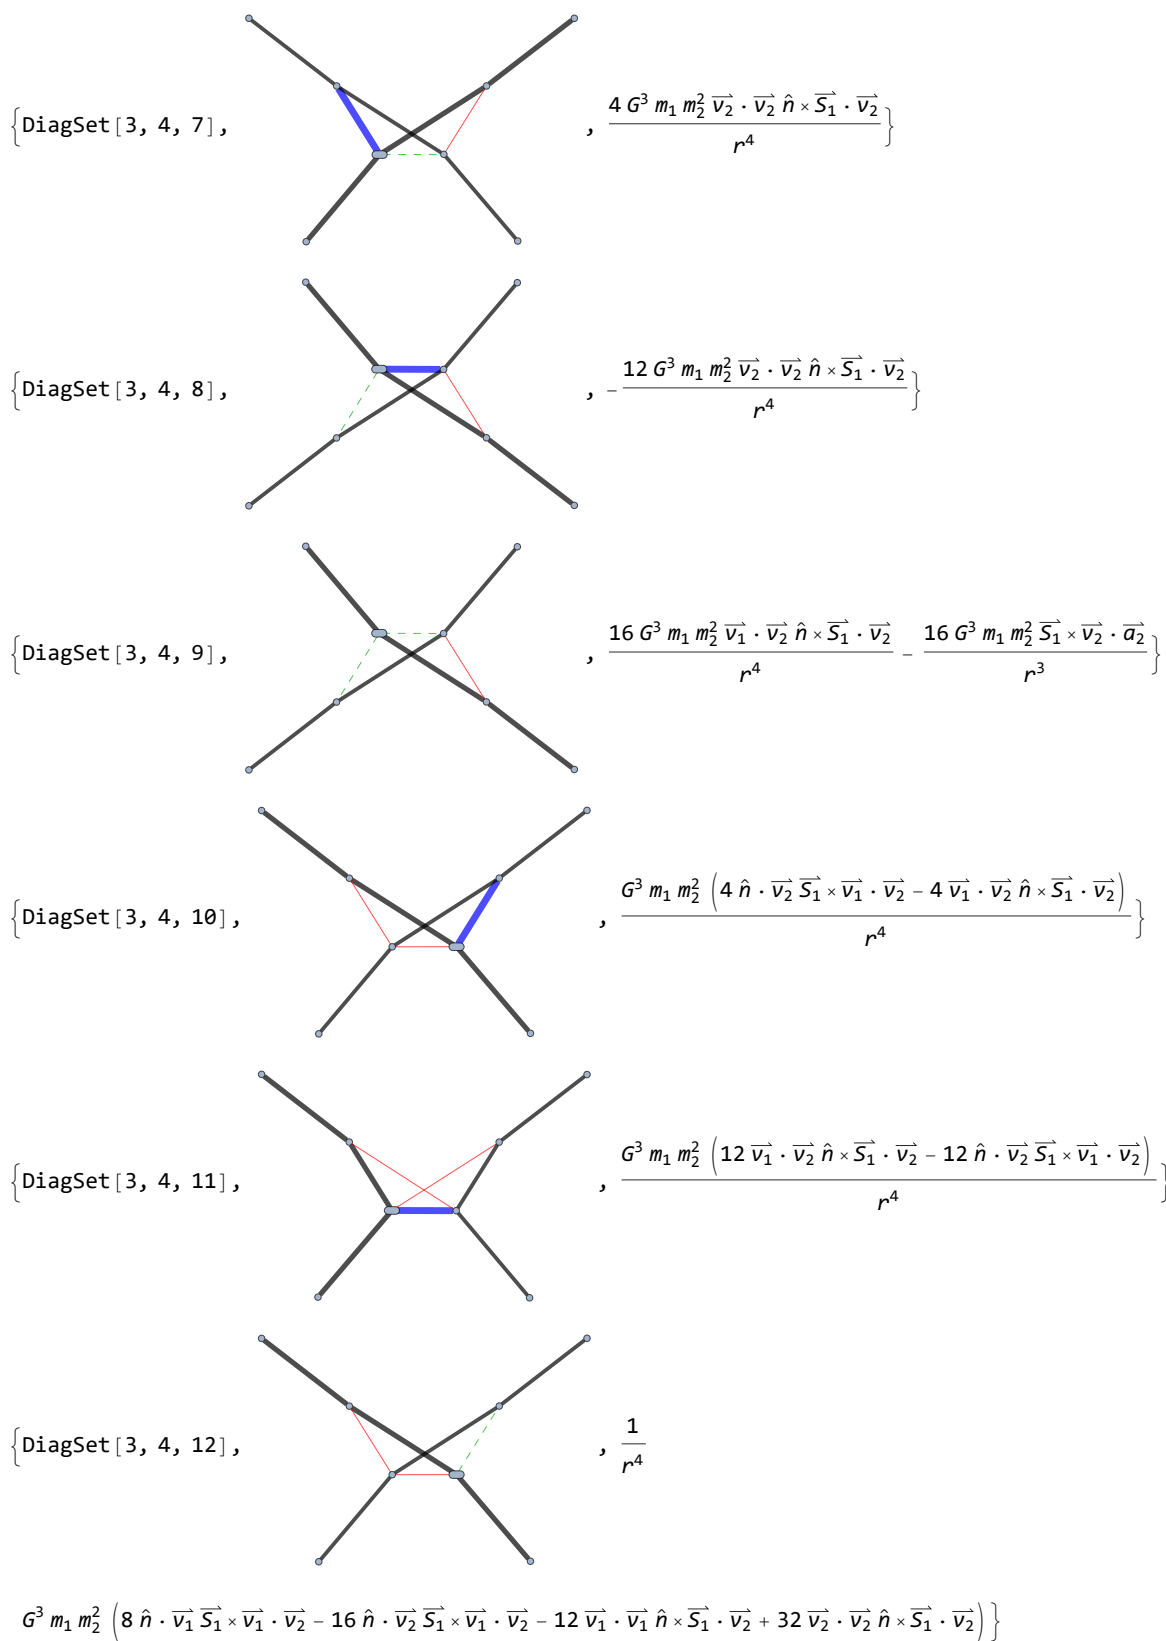  | $, \frac{G^3 m_1 m_2^2 \left( 4 \hat{n} \cdot \vec{v}_2 \vec{S}_1 \times \vec{v}_1 \cdot \vec{v}_2 - 4 \vec{v}_1 \cdot \vec{v}_2 \hat{n} \times \vec{S}_1 \cdot \vec{v}_2 \right)}{r^4} \}$   |
| $\{\text{DiagSet}[3, 4, 11],$ | 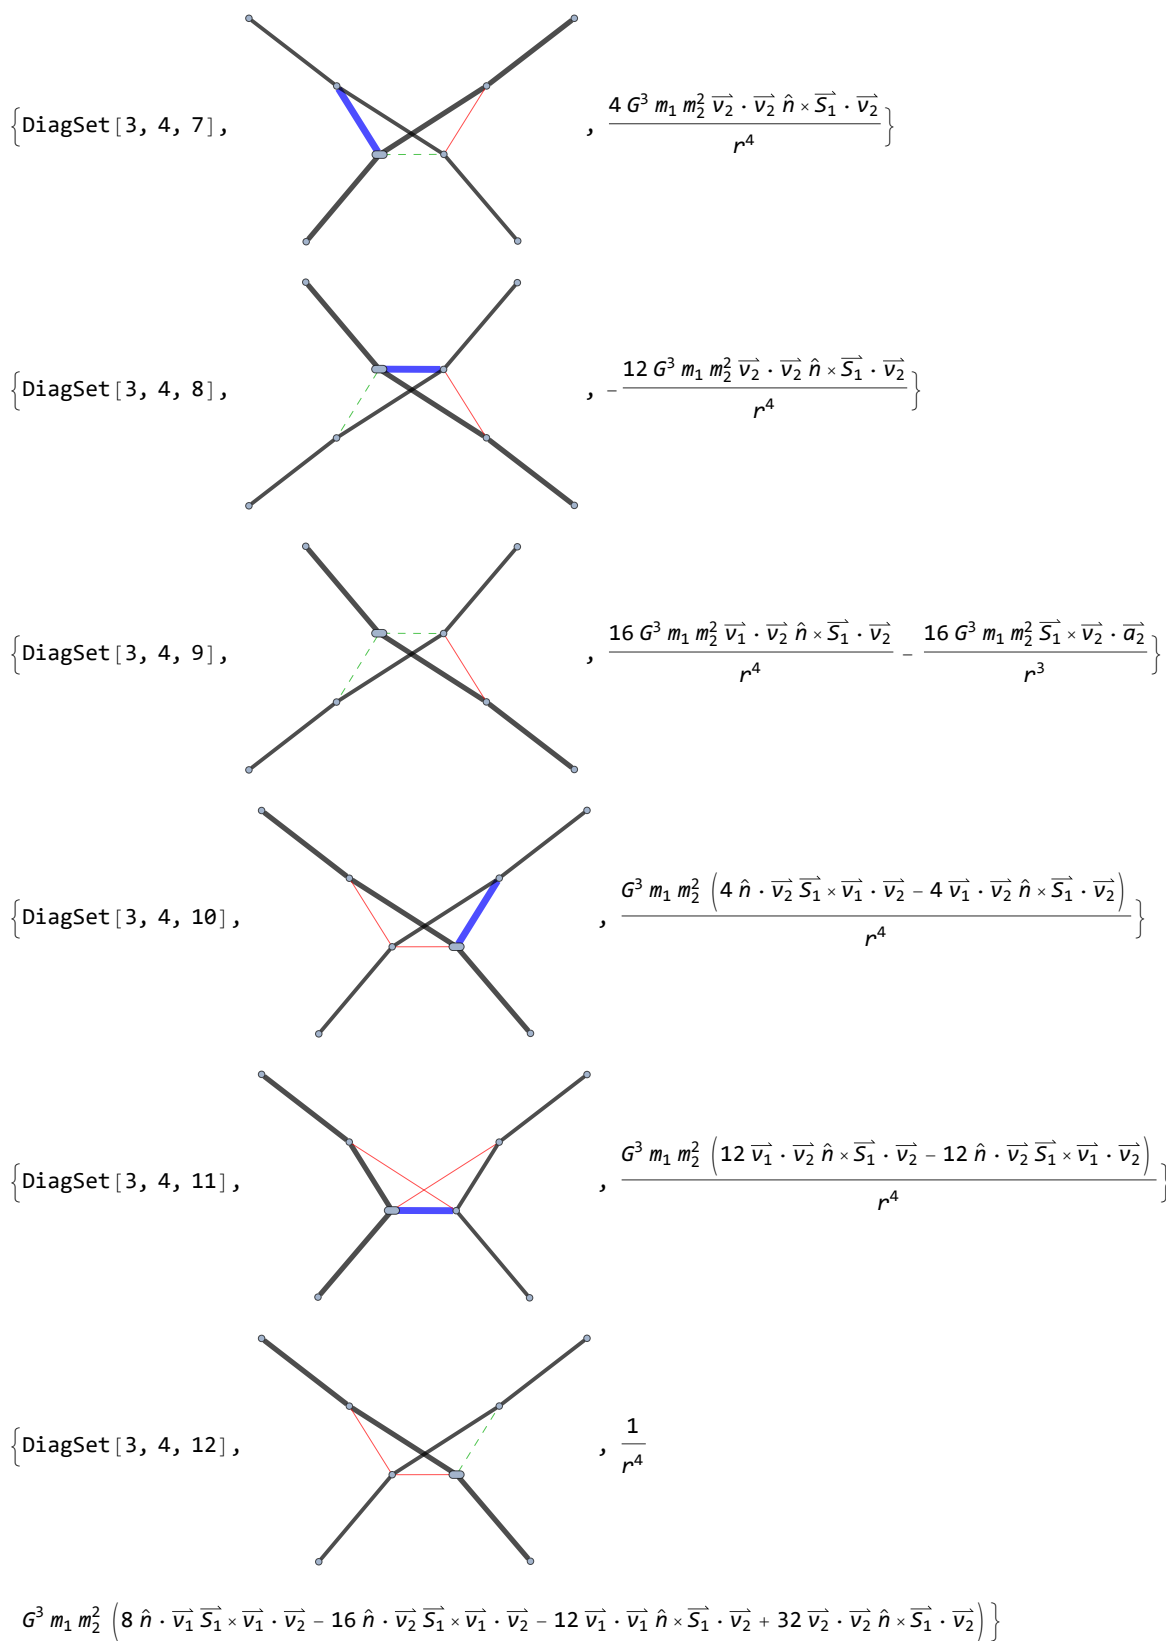 | $, \frac{G^3 m_1 m_2^2 \left( 12 \vec{v}_1 \cdot \vec{v}_2 \hat{n} \times \vec{S}_1 \cdot \vec{v}_2 - 12 \hat{n} \cdot \vec{v}_2 \vec{S}_1 \times \vec{v}_1 \cdot \vec{v}_2 \right)}{r^4} \}$ |
| $\{\text{DiagSet}[3, 4, 12],$ | 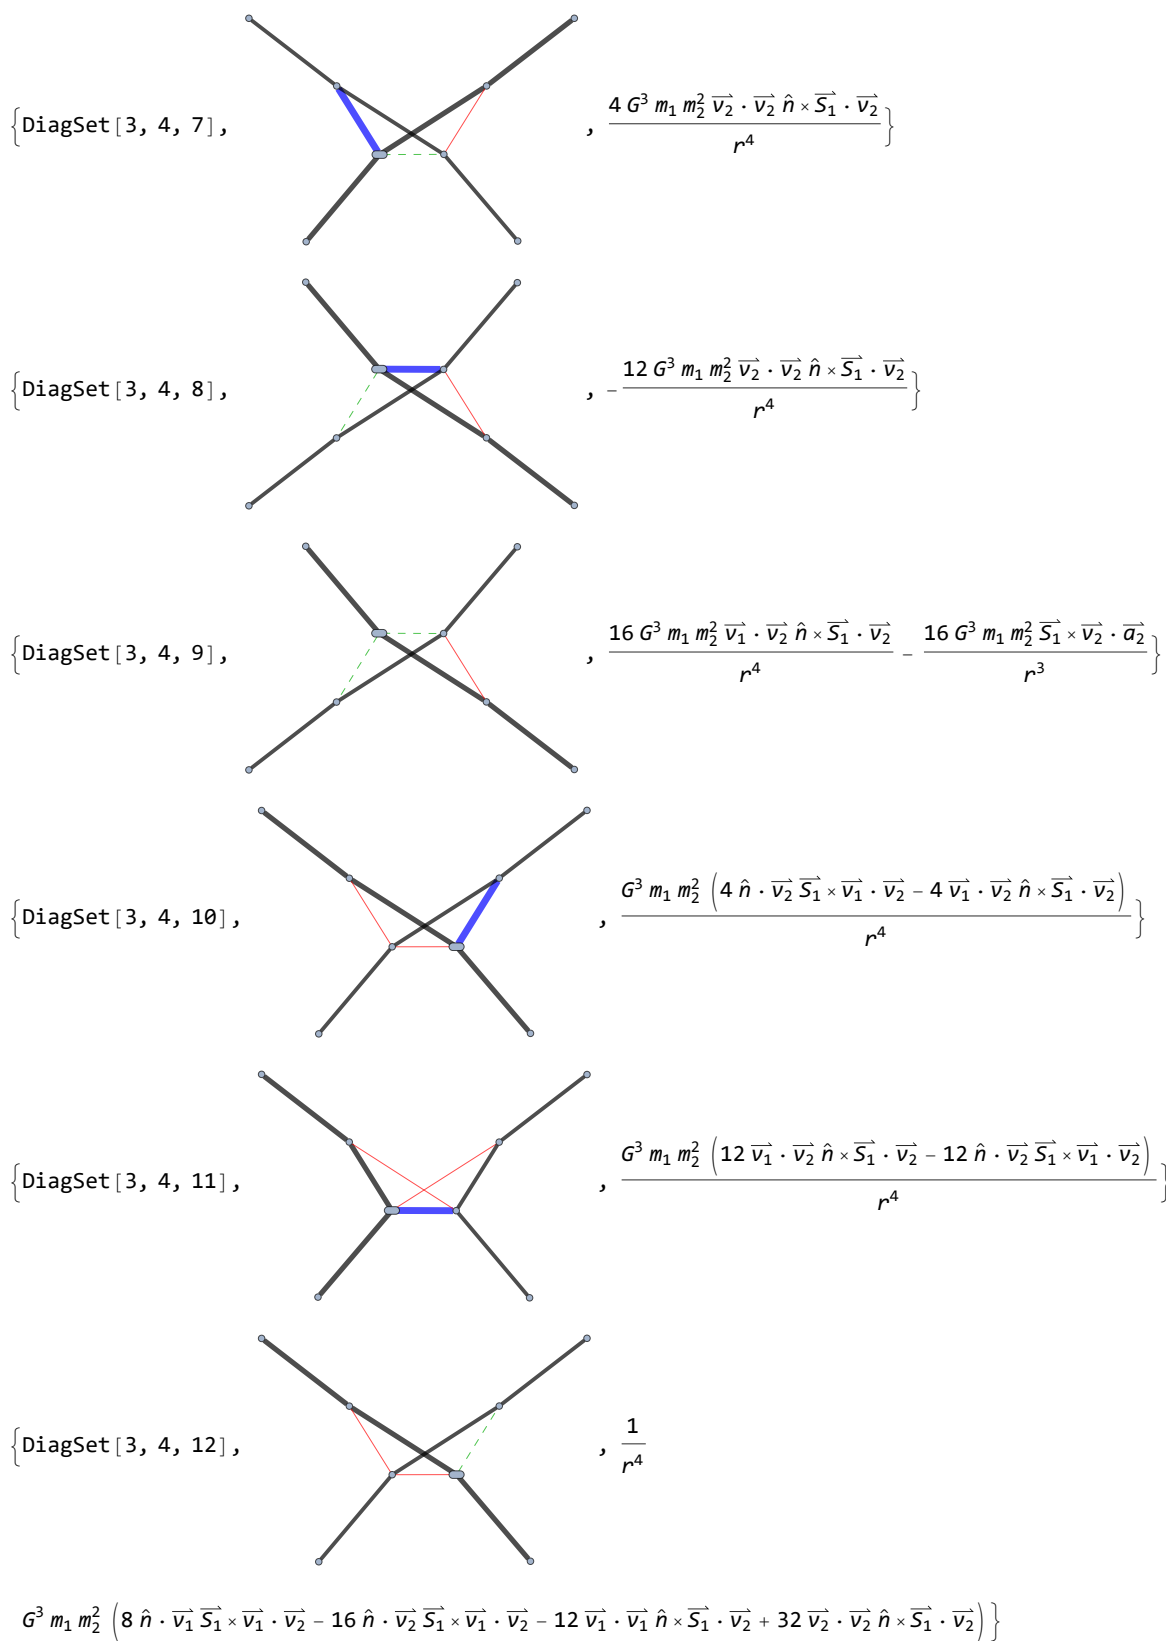 | $, \frac{1}{r^4} \}$                                                                                                                                                                          |

$$G^3 m_1 m_2^2 \left( 8 \hat{n} \cdot \vec{v}_1 \vec{S}_1 \times \vec{v}_1 \cdot \vec{v}_2 - 16 \hat{n} \cdot \vec{v}_2 \vec{S}_1 \times \vec{v}_1 \cdot \vec{v}_2 - 12 \vec{v}_1 \cdot \vec{v}_1 \hat{n} \times \vec{S}_1 \cdot \vec{v}_2 + 32 \vec{v}_2 \cdot \vec{v}_2 \hat{n} \times \vec{S}_1 \cdot \vec{v}_2 \right) \}$$

$$\left\{ \text{DiagSet}[3, 4, 13], \right. , \left. \frac{G^3 m_1 m_2^2 \left( -8 \hat{n} \cdot \vec{v}_2 \vec{S}_1 \times \vec{v}_1 \cdot \vec{v}_2 - 12 \vec{v}_1 \cdot \vec{v}_1 \hat{n} \times \vec{S}_1 \cdot \vec{v}_2 \right)}{r^4} \right\}$$
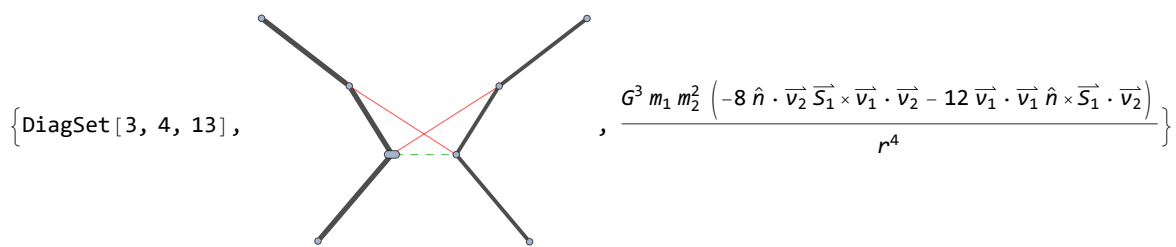

$$\left\{ \text{DiagSet}[3, 4, 14], \right. , \left. \frac{32 G^3 m_1 m_2^2 \vec{v}_1 \cdot \vec{v}_2 \hat{n} \times \vec{S}_1 \cdot \vec{v}_2}{r^4} \right\}$$
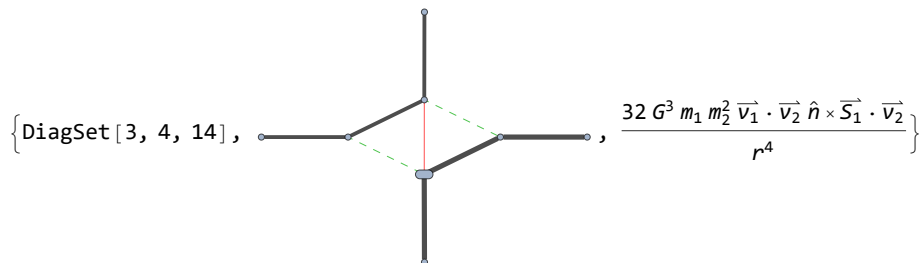

$$\left\{ \text{DiagSet}[3, 4, 15], \right. , \left. -\frac{8 G^3 m_1 m_2^2 \vec{S}_1 \times \vec{v}_1 \cdot \vec{a}_1}{r^3} - \frac{8 G^3 m_1 m_2^2 \vec{v}_1 \cdot \vec{v}_1 \hat{n} \times \vec{S}_1 \cdot \vec{v}_1}{r^4} \right\}$$
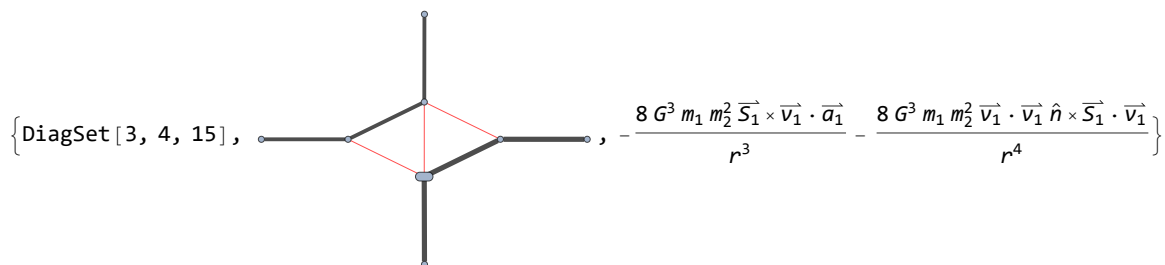

$$\left\{ \text{DiagSet}[3, 4, 16], \right. , \left. \right.$$
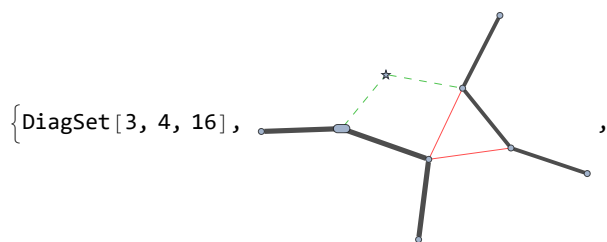

$$\frac{G^3 m_1 m_2^2 \left( \hat{n} \cdot \vec{v}_1 \hat{n} \times \vec{S}_1 \cdot \vec{a}_2 + \vec{S}_1 \times \vec{v}_1 \cdot \vec{a}_2 + 2 \hat{n} \cdot \vec{v}_1 \hat{n} \times \vec{S}_1 \cdot \vec{v}_2 - 3 \hat{n} \cdot \vec{v}_2 \hat{n} \times \vec{S}_1 \cdot \vec{v}_2 \right)}{r^3} - \frac{G^3 m_1 m_2^2 \hat{n} \times \vec{S}_1 \cdot \vec{a}_2}{r^2} + \frac{1}{r^4}$$

$$G^3 m_1 m_2^2 \left( -2 \left( \hat{n} \cdot \vec{v}_1 \right)^2 \hat{n} \times \vec{S}_1 \cdot \vec{v}_2 - 2 \hat{n} \cdot \vec{v}_1 \vec{S}_1 \times \vec{v}_1 \cdot \vec{v}_2 + 5 \hat{n} \cdot \vec{v}_2 \hat{n} \cdot \vec{v}_1 \hat{n} \times \vec{S}_1 \cdot \vec{v}_2 + 3 \hat{n} \cdot \vec{v}_2 \vec{S}_1 \times \vec{v}_1 \cdot \vec{v}_2 - \vec{v}_1 \cdot \vec{v}_2 \hat{n} \times \vec{S}_1 \cdot \vec{v}_2 \right) \}$$

$$\left\{ \text{DiagSet}[3, 4, 17], \right. , \left. \right.$$
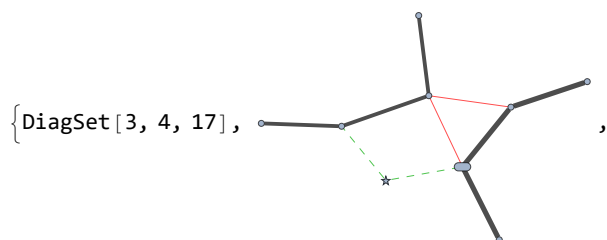

$$\frac{1}{r^3} G^3 m_1 m_2^2 \left( 12 \hat{n} \cdot \vec{v}_1 \hat{n} \times \vec{S}_1 \cdot \vec{a}_2 - 8 \hat{n} \cdot \vec{v}_2 \hat{n} \times \vec{S}_1 \cdot \vec{a}_2 + 4 \vec{S}_1 \times \vec{v}_1 \cdot \vec{a}_2 - 4 \hat{n} \cdot \vec{v}_2 \hat{n} \times \vec{S}_1 \cdot \vec{v}_2 \right) - \frac{4 G^3 m_1 m_2^2 \hat{n} \times \vec{S}_1 \cdot \vec{a}_2}{r^2} +$$

$$\frac{1}{r^4} G^3 m_1 m_2^2 \left( -8 \left( \hat{n} \cdot \vec{v}_2 \right)^2 \hat{n} \times \vec{S}_1 \cdot \vec{v}_2 + 4 \hat{n} \cdot \vec{v}_2 \vec{S}_1 \times \vec{v}_1 \cdot \vec{v}_2 + 20 \hat{n} \cdot \vec{v}_1 \hat{n} \cdot \vec{v}_2 \hat{n} \times \vec{S}_1 \cdot \vec{v}_2 - 4 \vec{v}_1 \cdot \vec{v}_2 \hat{n} \times \vec{S}_1 \cdot \vec{v}_2 \right) \}$$

{DiagSet[3, 4, 18],

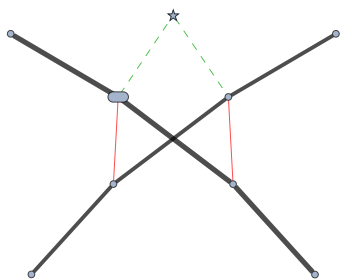

,

$$\frac{1}{r^3} G^3 m_1 m_2^2 \left( 8 \hat{n} \cdot \vec{v}_1 \hat{n} \times \vec{S}_1 \cdot \vec{a}_2 - 4 \hat{n} \cdot \vec{v}_2 \hat{n} \times \vec{S}_1 \cdot \vec{a}_2 + 4 \vec{S}_1 \times \vec{v}_1 \cdot \vec{a}_2 + 4 \hat{n} \cdot \vec{v}_1 \hat{n} \times \vec{S}_1 \cdot \vec{v}_2 - 8 \hat{n} \cdot \vec{v}_2 \hat{n} \times \vec{S}_1 \cdot \vec{v}_2 \right) -$$

$$\frac{4 G^3 m_1 m_2^2 \hat{n} \times \vec{S}_1 \cdot \vec{a}_2}{r^2} + \frac{1}{r^4} G^3 m_1 m_2^2 \left( -8 (\hat{n} \cdot \vec{v}_1)^2 \hat{n} \times \vec{S}_1 \cdot \vec{v}_2 - 4 \hat{n} \cdot \vec{v}_1 \vec{S}_1 \times \vec{v}_1 \cdot \vec{v}_2 + \right.$$

$$\left. 28 \hat{n} \cdot \vec{v}_2 \hat{n} \cdot \vec{v}_1 \hat{n} \times \vec{S}_1 \cdot \vec{v}_2 - 8 (\hat{n} \cdot \vec{v}_2)^2 \hat{n} \times \vec{S}_1 \cdot \vec{v}_2 + 8 \hat{n} \cdot \vec{v}_2 \vec{S}_1 \times \vec{v}_1 \cdot \vec{v}_2 - 4 \vec{v}_1 \cdot \vec{v}_2 \hat{n} \times \vec{S}_1 \cdot \vec{v}_2 \right) \Big\}$$

{DiagSet[3, 4, 19],

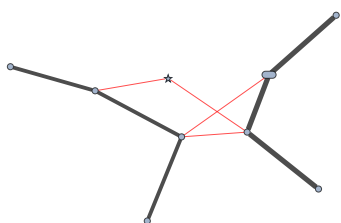

$$, \frac{G^3 m_1 m_2^2 \left( \hat{n} \cdot \vec{v}_2 \hat{n} \times \vec{S}_1 \cdot \vec{a}_1 + \hat{n} \cdot \vec{v}_2 \hat{n} \times \vec{S}_1 \cdot \vec{v}_1 \right)}{r^3} +$$

$$\frac{1}{r^4} G^3 m_1 m_2^2 \left( 4 (\hat{n} \cdot \vec{v}_2)^2 \hat{n} \times \vec{S}_1 \cdot \vec{v}_1 - \hat{n} \cdot \vec{v}_2 \vec{S}_1 \times \vec{v}_1 \cdot \vec{v}_2 - 5 \hat{n} \cdot \vec{v}_1 \hat{n} \cdot \vec{v}_2 \hat{n} \times \vec{S}_1 \cdot \vec{v}_1 + \vec{v}_1 \cdot \vec{v}_2 \hat{n} \times \vec{S}_1 \cdot \vec{v}_1 \right) \Big\}$$

{DiagSet[3, 4, 20],

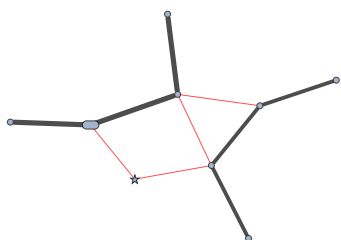

,

$$\frac{1}{r^3} G^3 m_1 m_2^2 \left( -2 \hat{n} \cdot \vec{v}_1 \hat{n} \times \vec{S}_1 \cdot \vec{a}_1 + 3 \hat{n} \cdot \vec{v}_2 \hat{n} \times \vec{S}_1 \cdot \vec{a}_1 - \vec{S}_1 \times \vec{a}_1 \cdot \vec{v}_2 - 2 \hat{n} \cdot \vec{v}_1 \hat{n} \times \vec{S}_1 \cdot \vec{v}_1 + 3 \hat{n} \cdot \vec{v}_2 \hat{n} \times \vec{S}_1 \cdot \vec{v}_1 - \left( \vec{S}_1 \times \vec{v}_1 \cdot \vec{v}_2 \right) \right) +$$

$$\frac{1}{r^4} G^3 m_1 m_2^2 \left( 2 (\hat{n} \cdot \vec{v}_1)^2 \hat{n} \times \vec{S}_1 \cdot \vec{v}_1 + \hat{n} \cdot \vec{v}_1 \vec{S}_1 \times \vec{v}_1 \cdot \vec{v}_2 - 5 \hat{n} \cdot \vec{v}_2 \hat{n} \cdot \vec{v}_1 \hat{n} \times \vec{S}_1 \cdot \vec{v}_1 + \vec{v}_1 \cdot \vec{v}_2 \hat{n} \times \vec{S}_1 \cdot \vec{v}_1 \right) \Big\}$$

{DiagSet[3, 4, 21],

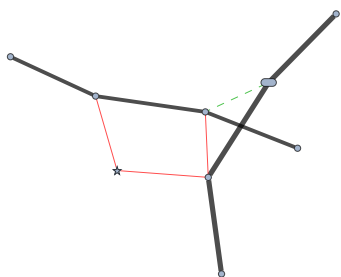

$$, \frac{G^3 m_1 m_2^2 \left( \hat{n} \cdot \vec{v}_2 \left( - \left( \hat{n} \times \vec{S}_1 \cdot \vec{v}_2 \right) \right) - \hat{n} \cdot \vec{v}_2 \hat{n} \times \vec{S}_1 \cdot \vec{a}_2 \right)}{r^3} +$$

$$\frac{1}{r^4} G^3 m_1 m_2^2 \left( -4 (\hat{n} \cdot \vec{v}_2)^2 \hat{n} \times \vec{S}_1 \cdot \vec{v}_2 + \hat{n} \cdot \vec{v}_2 \vec{S}_1 \times \vec{v}_1 \cdot \vec{v}_2 + 5 \hat{n} \cdot \vec{v}_1 \hat{n} \cdot \vec{v}_2 \hat{n} \times \vec{S}_1 \cdot \vec{v}_2 - \vec{v}_1 \cdot \vec{v}_2 \hat{n} \times \vec{S}_1 \cdot \vec{v}_2 \right) \Big\}$$

$$\left\{ \text{DiagSet}[3, 4, 22], \right. \quad \left. \frac{G^3 m_1 m_2^2 \left( 4 \hat{n} \cdot \vec{v}_1 \hat{n} \times \vec{S}_1 \cdot \vec{v}_2 - 4 \hat{n} \cdot \vec{v}_1 \hat{n} \times \vec{a}_2 \cdot \vec{S}_1 \right)}{r^3} + \frac{1}{r^4} \right.$$
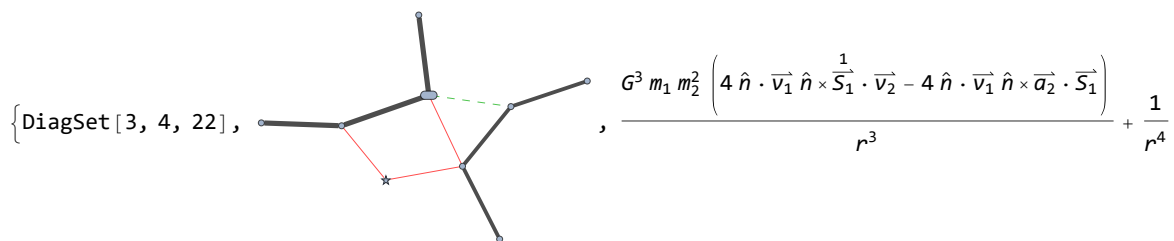

$$\left. G^3 m_1 m_2^2 \left( -16 (\hat{n} \cdot \vec{v}_1)^2 \hat{n} \times \vec{S}_1 \cdot \vec{v}_2 - 4 \hat{n} \cdot \vec{v}_1 \vec{S}_1 \times \vec{v}_1 \cdot \vec{v}_2 + 20 \hat{n} \cdot \vec{v}_2 \hat{n} \cdot \vec{v}_1 \hat{n} \times \vec{S}_1 \cdot \vec{v}_2 - 4 \vec{v}_1 \cdot \vec{v}_2 \hat{n} \times \vec{S}_1 \cdot \vec{v}_2 \right) \right\}$$

$$\left\{ \text{DiagSet}[3, 4, 23], \right. \quad \left. \frac{G^3 m_1 m_2^2 \left( \hat{n} \cdot \vec{v}_2 \left( - \left( \hat{n} \times \vec{S}_1 \cdot \vec{v}_1 \right) \right) - \hat{n} \cdot \vec{v}_2 \hat{n} \times \vec{S}_1 \cdot \vec{a}_1 \right)}{r^3} + \right.$$
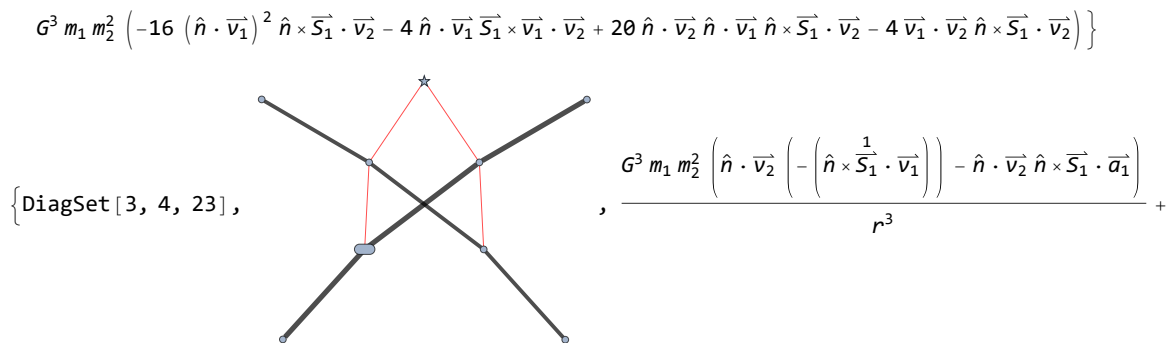

$$\left. \frac{1}{r^4} G^3 m_1 m_2^2 \left( -2 (\hat{n} \cdot \vec{v}_2)^2 \hat{n} \times \vec{S}_1 \cdot \vec{v}_1 + \hat{n} \cdot \vec{v}_2 \vec{S}_1 \times \vec{v}_1 \cdot \vec{v}_2 + \hat{n} \cdot \vec{v}_1 \hat{n} \cdot \vec{v}_2 \hat{n} \times \vec{S}_1 \cdot \vec{v}_1 + \vec{v}_1 \cdot \vec{v}_2 \hat{n} \times \vec{S}_1 \cdot \vec{v}_1 \right) \right\}$$

$$\left\{ \text{DiagSet}[3, 4, 24], \right. \quad \left. \frac{G^3 m_1 m_2^2 \left( \hat{n} \cdot \vec{v}_2 \hat{n} \times \vec{S}_1 \cdot \vec{a}_2 + \hat{n} \cdot \vec{v}_2 \hat{n} \times \vec{S}_1 \cdot \vec{v}_2 \right)}{r^3} + \right.$$
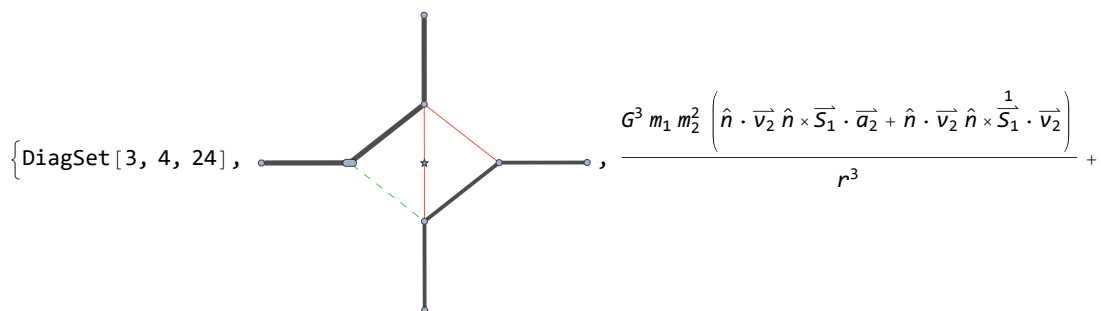

$$\left. \frac{1}{r^4} G^3 m_1 m_2^2 \left( 2 (\hat{n} \cdot \vec{v}_2)^2 \hat{n} \times \vec{S}_1 \cdot \vec{v}_2 - \hat{n} \cdot \vec{v}_2 \vec{S}_1 \times \vec{v}_1 \cdot \vec{v}_2 - \hat{n} \cdot \vec{v}_1 \hat{n} \cdot \vec{v}_2 \hat{n} \times \vec{S}_1 \cdot \vec{v}_2 - \vec{v}_1 \cdot \vec{v}_2 \hat{n} \times \vec{S}_1 \cdot \vec{v}_2 \right) \right\}$$

$$\left\{ \text{DiagSet}[3, 4, 25], \right. \quad \left. \frac{G^3 m_1 m_2^2 \left( 4 \hat{n} \cdot \vec{v}_1 \hat{n} \times \vec{a}_2 \cdot \vec{S}_1 - 4 \hat{n} \cdot \vec{v}_1 \hat{n} \times \vec{S}_1 \cdot \vec{v}_2 \right)}{r^3} + \right.$$
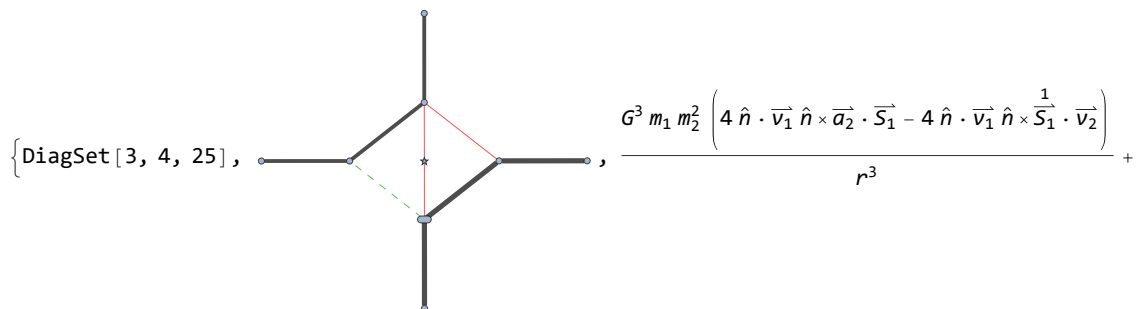

$$\left. \frac{1}{r^4} G^3 m_1 m_2^2 \left( 8 (\hat{n} \cdot \vec{v}_1)^2 \hat{n} \times \vec{S}_1 \cdot \vec{v}_2 + 4 \hat{n} \cdot \vec{v}_1 \vec{S}_1 \times \vec{v}_1 \cdot \vec{v}_2 - 4 \hat{n} \cdot \vec{v}_2 \hat{n} \cdot \vec{v}_1 \hat{n} \times \vec{S}_1 \cdot \vec{v}_2 - 4 \vec{v}_1 \cdot \vec{v}_2 \hat{n} \times \vec{S}_1 \cdot \vec{v}_2 \right) \right\}$$

$$\left\{ \text{DiagSet}[3, 4, 26], \right. \quad \left. \frac{G^3 m_1 m_2^2 \left( 4 \hat{n} \cdot \vec{v}_1 \hat{n} \times \vec{S}_1 \cdot \vec{a}_2 + 4 \hat{n} \cdot \vec{v}_1 \hat{n} \times \vec{S}_1 \cdot \vec{v}_2 \right)}{r^3} + \frac{1}{r^4} \right.$$
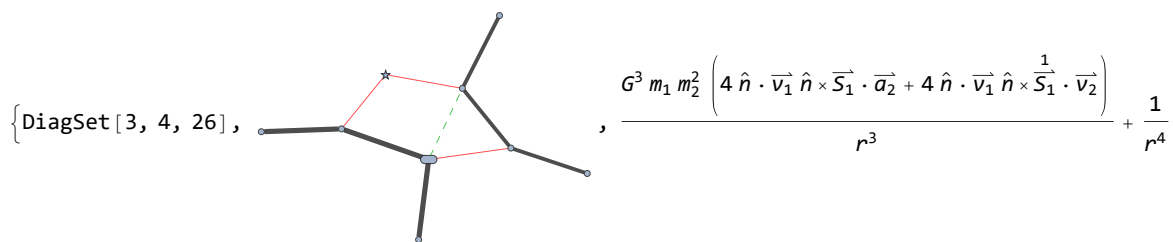

$$G^3 m_1 m_2^2 \left( -16 (\hat{n} \cdot \vec{v}_1)^2 \hat{n} \times \vec{S}_1 \cdot \vec{v}_2 - 4 \hat{n} \cdot \vec{v}_1 \vec{S}_1 \times \vec{v}_1 \cdot \vec{v}_2 + 20 \hat{n} \cdot \vec{v}_2 \hat{n} \cdot \vec{v}_1 \hat{n} \times \vec{S}_1 \cdot \vec{v}_2 - 4 \vec{v}_1 \cdot \vec{v}_2 \hat{n} \times \vec{S}_1 \cdot \vec{v}_2 \right) \Big\}$$

$$\left\{ \text{DiagSet}[3, 4, 27], \right. \left. \frac{G^3 m_1 m_2^2 \left( -4 \hat{n} \cdot \vec{v}_2 \hat{n} \times \vec{S}_1 \cdot \vec{v}_2 - 4 \hat{n} \cdot \vec{v}_2 \hat{n} \times \vec{S}_1 \cdot \vec{v}_2 \right)}{r^3} + \right.$$
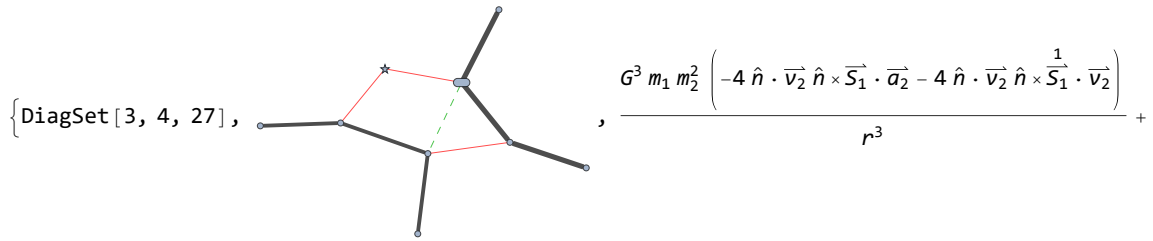

$$\frac{1}{r^4} G^3 m_1 m_2^2 \left( -16 (\hat{n} \cdot \vec{v}_2)^2 \hat{n} \times \vec{S}_1 \cdot \vec{v}_2 + 4 \hat{n} \cdot \vec{v}_2 \vec{S}_1 \times \vec{v}_1 \cdot \vec{v}_2 + 20 \hat{n} \cdot \vec{v}_1 \hat{n} \cdot \vec{v}_2 \hat{n} \times \vec{S}_1 \cdot \vec{v}_2 - 4 \vec{v}_1 \cdot \vec{v}_2 \hat{n} \times \vec{S}_1 \cdot \vec{v}_2 \right) \Big\}$$

$$\left\{ \text{DiagSet}[3, 5, 1], \right.$$
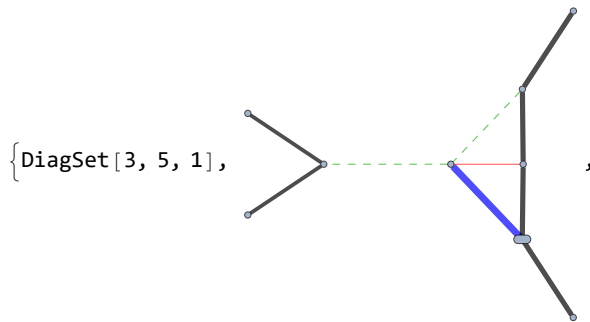

$$\frac{G^3 m_1^2 m_2 \left( \frac{16}{5} \hat{n} \cdot \vec{v}_1 \vec{S}_1 \times \vec{v}_1 \cdot \vec{v}_2 + \frac{64}{5} \vec{v}_1 \cdot \vec{v}_1 \hat{n} \times \vec{S}_1 \cdot \vec{v}_2 - 16 \vec{v}_1 \cdot \vec{v}_2 \hat{n} \times \vec{S}_1 \cdot \vec{v}_1 \right)}{r^4} \Big\}$$

$$\left\{ \text{DiagSet}[3, 5, 2], \right. \left. , 0 \right\}$$
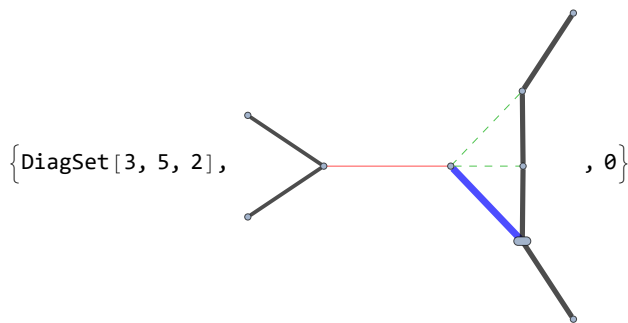

$$\left\{ \text{DiagSet}[3, 5, 3], \right. \left. , \frac{1}{r^4} \right.$$
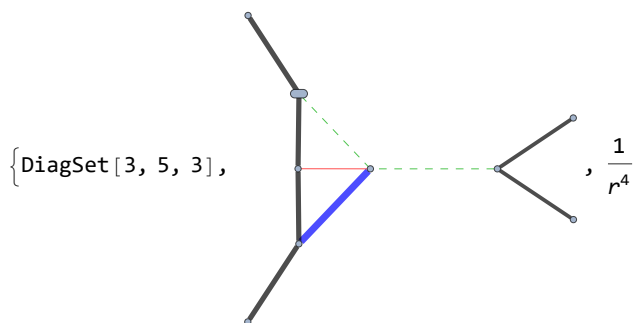

$$G^3 m_1^2 m_2 \left( \frac{48 (\hat{n} \cdot \vec{v}_1)^2 \hat{n} \times \vec{S}_1 \cdot \vec{v}_2 + \frac{96}{5} \hat{n} \cdot \vec{v}_1 \vec{S}_1 \times \vec{v}_1 \cdot \vec{v}_2 - \frac{48}{5} \vec{v}_1 \cdot \vec{v}_1 \hat{n} \times \vec{S}_1 \cdot \vec{v}_2}{\epsilon_d} - \right.$$

$$144 \log\left(\frac{r}{R_0}\right) (\hat{n} \cdot \vec{v}_1)^2 \hat{n} \times \vec{S}_1 \cdot \vec{v}_2 - \frac{288}{5} \log\left(\frac{r}{R_0}\right) \hat{n} \cdot \vec{v}_1 \vec{S}_1 \times \vec{v}_1 \cdot \vec{v}_2 + \frac{144}{5} \log\left(\frac{r}{R_0}\right) \vec{v}_1 \cdot \vec{v}_1 \hat{n} \times \vec{S}_1 \cdot \vec{v}_2 +$$

$$64 \left( \hat{n} \cdot \vec{v}_1 \right)^2 \hat{n} \times \vec{S}_1 \cdot \vec{v}_2 + \frac{672}{25} \hat{n} \cdot \vec{v}_1 \vec{S}_1 \times \vec{v}_1 \cdot \vec{v}_2 - \frac{336}{25} \vec{v}_1 \cdot \vec{v}_1 \hat{n} \times \vec{S}_1 \cdot \vec{v}_2 + \frac{32}{5} \vec{v}_1 \cdot \vec{v}_2 \hat{n} \times \vec{S}_1 \cdot \vec{v}_1 \right) \Bigg\}$$

$$\left\{ \text{DiagSet}[3, 5, 4], \frac{1}{r^4} \right\}$$

$$G^3 m_1^2 m_2 \left( \frac{-\frac{48}{7} \left( \hat{n} \cdot \vec{v}_2 \right)^2 \hat{n} \times \vec{S}_1 \cdot \vec{v}_1 + \frac{96}{35} \hat{n} \cdot \vec{v}_2 \vec{S}_1 \times \vec{v}_1 \cdot \vec{v}_2 + \frac{48}{35} \vec{v}_2 \cdot \vec{v}_2 \hat{n} \times \vec{S}_1 \cdot \vec{v}_1}{\epsilon_d} + \right. \\ \left. \frac{144}{7} \log\left(\frac{r}{R_0}\right) \left( \hat{n} \cdot \vec{v}_2 \right)^2 \hat{n} \times \vec{S}_1 \cdot \vec{v}_1 - \frac{288}{35} \log\left(\frac{r}{R_0}\right) \hat{n} \cdot \vec{v}_2 \vec{S}_1 \times \vec{v}_1 \cdot \vec{v}_2 - \frac{144}{35} \log\left(\frac{r}{R_0}\right) \vec{v}_2 \cdot \vec{v}_2 \hat{n} \times \vec{S}_1 \cdot \vec{v}_1 - \right. \\ \left. \frac{640}{49} \left( \hat{n} \cdot \vec{v}_2 \right)^2 \hat{n} \times \vec{S}_1 \cdot \vec{v}_1 + \frac{8864}{1225} \hat{n} \cdot \vec{v}_2 \vec{S}_1 \times \vec{v}_1 \cdot \vec{v}_2 - \frac{16}{5} \vec{v}_1 \cdot \vec{v}_2 \hat{n} \times \vec{S}_1 \cdot \vec{v}_2 + \frac{4432}{1225} \vec{v}_2 \cdot \vec{v}_2 \hat{n} \times \vec{S}_1 \cdot \vec{v}_1 \right) \Bigg\}$$

$$\left\{ \text{DiagSet}[3, 5, 5], \frac{1}{r^4} \right\}$$

$$G^3 m_1^2 m_2 \left( \frac{\frac{48}{35} \vec{v}_1 \cdot \vec{v}_1 \hat{n} \times \vec{S}_1 \cdot \vec{v}_1 - \frac{48}{7} \left( \hat{n} \cdot \vec{v}_1 \right)^2 \hat{n} \times \vec{S}_1 \cdot \vec{v}_1}{\epsilon_d} + \frac{144}{7} \log\left(\frac{r}{R_0}\right) \left( \hat{n} \cdot \vec{v}_1 \right)^2 \hat{n} \times \vec{S}_1 \cdot \vec{v}_1 - \right. \\ \left. \frac{144}{35} \log\left(\frac{r}{R_0}\right) \vec{v}_1 \cdot \vec{v}_1 \hat{n} \times \vec{S}_1 \cdot \vec{v}_1 - \frac{640}{49} \left( \hat{n} \cdot \vec{v}_1 \right)^2 \hat{n} \times \vec{S}_1 \cdot \vec{v}_1 + \frac{512}{1225} \vec{v}_1 \cdot \vec{v}_1 \hat{n} \times \vec{S}_1 \cdot \vec{v}_1 \right) \Bigg\}$$

$$\left\{ \text{DiagSet}[3, 5, 6], \frac{G^3 m_2^3 \left( \frac{64}{5} \vec{v}_2 \cdot \vec{v}_2 \hat{n} \times \vec{S}_1 \cdot \vec{v}_1 - 16 \vec{v}_1 \cdot \vec{v}_2 \hat{n} \times \vec{S}_1 \cdot \vec{v}_2 \right)}{r^4} \right\}$$

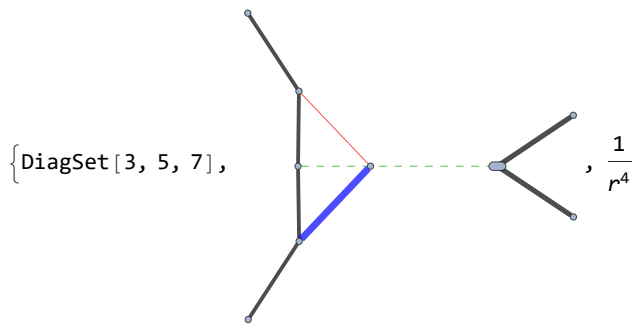

$$G^3 m_2^3 \left( \frac{80 (\hat{n} \cdot \vec{v}_2)^2 \hat{n} \times \vec{S}_1 \cdot \vec{v}_2 - 16 \vec{v}_2 \cdot \vec{v}_2 \hat{n} \times \vec{S}_1 \cdot \vec{v}_2}{\epsilon_d} - 240 \log\left(\frac{r}{R_0}\right) (\hat{n} \cdot \vec{v}_2)^2 \hat{n} \times \vec{S}_1 \cdot \vec{v}_2 + \right. \\ \left. 48 \log\left(\frac{r}{R_0}\right) \vec{v}_2 \cdot \vec{v}_2 \hat{n} \times \vec{S}_1 \cdot \vec{v}_2 + 128 (\hat{n} \cdot \vec{v}_2)^2 \hat{n} \times \vec{S}_1 \cdot \vec{v}_2 - 16 \vec{v}_2 \cdot \vec{v}_2 \hat{n} \times \vec{S}_1 \cdot \vec{v}_2 \right) \Big\}$$

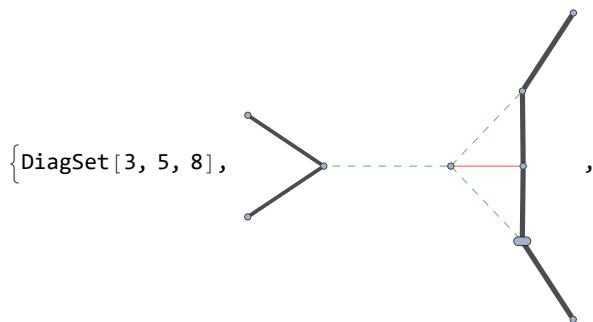

$$\frac{1}{r^3} m_1^2 m_2 \left( \frac{64}{5} \log\left(\frac{r}{R_0}\right) \vec{S}_1 \times \vec{a}_1 \cdot \vec{v}_2 + \frac{64}{25} \vec{S}_1 \times \vec{a}_1 \cdot \vec{v}_2 - \frac{32}{25} \vec{S}_1 \times \vec{v}_1 \cdot \vec{a}_2 - \frac{224}{25} \hat{n} \times \vec{S}_1 \cdot \vec{v}_2 \hat{n} \cdot \vec{a}_1 + \frac{288}{25} \hat{n} \times \vec{S}_1 \cdot \vec{v}_1 \hat{n} \cdot \vec{a}_2 + \right. \\ \frac{288}{25} \hat{n} \times \vec{S}_1 \cdot \vec{v}_2 \hat{n} \cdot \vec{v}_1 - \frac{288}{25} \hat{n} \times \vec{S}_1 \cdot \vec{a}_2 \hat{n} \cdot \vec{v}_1 + \frac{288}{25} \hat{n} \times \vec{S}_1 \cdot \vec{v}_1 \hat{n} \cdot \vec{v}_2 + \frac{224}{25} \hat{n} \times \vec{S}_1 \cdot \vec{a}_1 \hat{n} \cdot \vec{v}_2 + \\ \frac{128}{5} \vec{S}_1 \times \vec{v}_1 \cdot \vec{a}_2 \log\left(\frac{r}{R_0}\right) + \frac{96}{5} \hat{n} \times \vec{S}_1 \cdot \vec{v}_2 \hat{n} \cdot \vec{a}_1 \log\left(\frac{r}{R_0}\right) - \frac{192}{5} \hat{n} \times \vec{S}_1 \cdot \vec{v}_1 \hat{n} \cdot \vec{a}_2 \log\left(\frac{r}{R_0}\right) - \\ \frac{192}{5} \hat{n} \times \vec{S}_1 \cdot \vec{v}_2 \hat{n} \cdot \vec{v}_1 \log\left(\frac{r}{R_0}\right) + \frac{192}{5} \hat{n} \times \vec{S}_1 \cdot \vec{a}_2 \hat{n} \cdot \vec{v}_1 \log\left(\frac{r}{R_0}\right) - \frac{192}{5} \hat{n} \times \vec{S}_1 \cdot \vec{v}_1 \hat{n} \cdot \vec{v}_2 \log\left(\frac{r}{R_0}\right) - \\ \frac{96}{5} \hat{n} \times \vec{S}_1 \cdot \vec{a}_1 \hat{n} \cdot \vec{v}_2 \log\left(\frac{r}{R_0}\right) + \frac{1}{\epsilon_d} \left( -\frac{64}{15} \vec{S}_1 \times \vec{a}_1 \cdot \vec{v}_2 - \frac{128}{15} \vec{S}_1 \times \vec{v}_1 \cdot \vec{a}_2 - \frac{32}{5} \hat{n} \times \vec{S}_1 \cdot \vec{v}_2 \hat{n} \cdot \vec{a}_1 + \frac{64}{5} \hat{n} \times \vec{S}_1 \cdot \vec{v}_1 \hat{n} \cdot \vec{a}_2 + \right. \\ \left. \frac{64}{5} \hat{n} \times \vec{S}_1 \cdot \vec{v}_2 \hat{n} \cdot \vec{v}_1 - \frac{64}{5} \hat{n} \times \vec{S}_1 \cdot \vec{a}_2 \hat{n} \cdot \vec{v}_1 + \frac{64}{5} \hat{n} \times \vec{S}_1 \cdot \vec{v}_1 \hat{n} \cdot \vec{v}_2 + \frac{32}{5} \hat{n} \times \vec{S}_1 \cdot \vec{a}_1 \hat{n} \cdot \vec{v}_2 \right) \Big) G^3 + \\ \frac{1}{r^4} m_1^2 m_2 \left( -32 \hat{n} \times \vec{S}_1 \cdot \vec{v}_2 (\hat{n} \cdot \vec{v}_1)^2 + 96 \hat{n} \times \vec{S}_1 \cdot \vec{v}_2 \log\left(\frac{r}{R_0}\right) (\hat{n} \cdot \vec{v}_1)^2 - \frac{8864 \vec{S}_1 \times \vec{v}_1 \cdot \vec{v}_2 \hat{n} \cdot \vec{v}_1}{1225} - \right. \\ \frac{3424}{49} \hat{n} \times \vec{S}_1 \cdot \vec{v}_1 \hat{n} \cdot \vec{v}_2 \hat{n} \cdot \vec{v}_1 - 96 \hat{n} \times \vec{S}_1 \cdot \vec{v}_2 \hat{n} \cdot \vec{v}_2 \hat{n} \cdot \vec{v}_1 + \frac{288}{35} \vec{S}_1 \times \vec{v}_1 \cdot \vec{v}_2 \log\left(\frac{r}{R_0}\right) \hat{n} \cdot \vec{v}_1 + \\ \frac{1056}{7} \hat{n} \times \vec{S}_1 \cdot \vec{v}_1 \hat{n} \cdot \vec{v}_2 \log\left(\frac{r}{R_0}\right) \hat{n} \cdot \vec{v}_1 + 192 \hat{n} \times \vec{S}_1 \cdot \vec{v}_2 \hat{n} \cdot \vec{v}_2 \log\left(\frac{r}{R_0}\right) \hat{n} \cdot \vec{v}_1 + 96 \hat{n} \times \vec{S}_1 \cdot \vec{v}_1 (\hat{n} \cdot \vec{v}_2)^2 - \\ \frac{1024}{25} \vec{S}_1 \times \vec{v}_1 \cdot \vec{v}_2 \hat{n} \cdot \vec{v}_2 + \frac{64}{25} \hat{n} \times \vec{S}_1 \cdot \vec{v}_2 \vec{v}_1 \cdot \vec{v}_1 + \frac{20928 \hat{n} \times \vec{S}_1 \cdot \vec{v}_1 \vec{v}_1 \cdot \vec{v}_2}{1225} + \frac{288}{25} \hat{n} \times \vec{S}_1 \cdot \vec{v}_2 \vec{v}_1 \cdot \vec{v}_2 - \\ \frac{288}{25} \hat{n} \times \vec{S}_1 \cdot \vec{v}_1 \vec{v}_2 \cdot \vec{v}_2 - 192 \hat{n} \times \vec{S}_1 \cdot \vec{v}_1 (\hat{n} \cdot \vec{v}_2)^2 \log\left(\frac{r}{R_0}\right) + \frac{576}{5} \vec{S}_1 \times \vec{v}_1 \cdot \vec{v}_2 \hat{n} \cdot \vec{v}_2 \log\left(\frac{r}{R_0}\right) - \\ \frac{96}{5} \hat{n} \times \vec{S}_1 \cdot \vec{v}_2 \vec{v}_1 \cdot \vec{v}_1 \log\left(\frac{r}{R_0}\right) - \frac{1056}{35} \hat{n} \times \vec{S}_1 \cdot \vec{v}_1 \vec{v}_1 \cdot \vec{v}_2 \log\left(\frac{r}{R_0}\right) - \frac{192}{5} \hat{n} \times \vec{S}_1 \cdot \vec{v}_2 \vec{v}_1 \cdot \vec{v}_2 \log\left(\frac{r}{R_0}\right) + \right.$$

$$\begin{aligned} & \frac{192}{5} \hat{n} \times \vec{S}_1 \cdot \vec{v}_1 \vec{v}_2 \cdot \vec{v}_2 \log\left(\frac{r}{R_\theta}\right) + \frac{1}{\epsilon_d} \left( -32 \hat{n} \times \vec{S}_1 \cdot \vec{v}_2 (\hat{n} \cdot \vec{v}_1)^2 - \frac{96}{35} \vec{S}_1 \times \vec{v}_1 \cdot \vec{v}_2 \hat{n} \cdot \vec{v}_1 - \right. \\ & \quad \frac{352}{7} \hat{n} \times \vec{S}_1 \cdot \vec{v}_1 \hat{n} \cdot \vec{v}_2 \hat{n} \cdot \vec{v}_1 - 64 \hat{n} \times \vec{S}_1 \cdot \vec{v}_2 \hat{n} \cdot \vec{v}_2 \hat{n} \cdot \vec{v}_1 + 64 \hat{n} \times \vec{S}_1 \cdot \vec{v}_1 (\hat{n} \cdot \vec{v}_2)^2 - \frac{192}{5} \vec{S}_1 \times \vec{v}_1 \cdot \vec{v}_2 \hat{n} \cdot \vec{v}_2 + \\ & \quad \left. \frac{32}{5} \hat{n} \times \vec{S}_1 \cdot \vec{v}_2 \vec{v}_1 \cdot \vec{v}_1 + \frac{352}{35} \hat{n} \times \vec{S}_1 \cdot \vec{v}_1 \vec{v}_1 \cdot \vec{v}_2 + \frac{64}{5} \hat{n} \times \vec{S}_1 \cdot \vec{v}_2 \vec{v}_1 \cdot \vec{v}_2 - \frac{64}{5} \hat{n} \times \vec{S}_1 \cdot \vec{v}_1 \vec{v}_2 \cdot \vec{v}_2 \right) \Bigg\} \mathcal{G}^3 \Bigg\} \end{aligned}$$

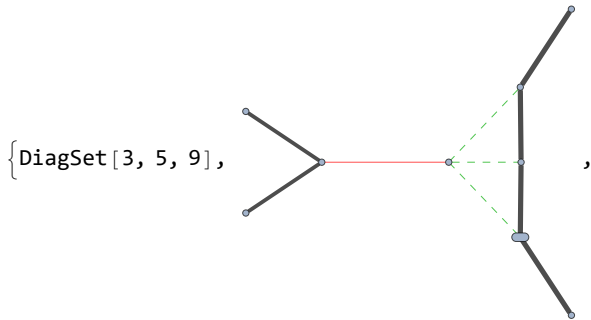

$$\begin{aligned} & \frac{1}{r^3} G^3 m_1^2 m_2 \left( \frac{\frac{64}{5} \hat{n} \cdot \vec{a}_1 \hat{n} \times \vec{S}_1 \cdot \vec{v}_1 - \frac{64}{5} \hat{n} \cdot \vec{v}_1 \hat{n} \times \vec{S}_1 \cdot \vec{a}_1 - \frac{128}{15} \vec{S}_1 \times \vec{v}_1 \cdot \vec{a}_1 - \frac{32}{5} \hat{n} \cdot \vec{v}_1 \hat{n} \times \vec{S}_1 \cdot \vec{v}_1}{\epsilon_d} - \right. \\ & \quad \frac{192}{5} \log\left(\frac{r}{R_\theta}\right) \hat{n} \cdot \vec{a}_1 \hat{n} \times \vec{S}_1 \cdot \vec{v}_1 + \frac{192}{5} \log\left(\frac{r}{R_\theta}\right) \hat{n} \cdot \vec{v}_1 \hat{n} \times \vec{S}_1 \cdot \vec{a}_1 + \frac{288}{25} \hat{n} \cdot \vec{a}_1 \hat{n} \times \vec{S}_1 \cdot \vec{v}_1 - \frac{288}{25} \hat{n} \cdot \vec{v}_1 \hat{n} \times \vec{S}_1 \cdot \vec{a}_1 + \\ & \quad \left. \frac{128}{5} \log\left(\frac{r}{R_\theta}\right) \vec{S}_1 \times \vec{v}_1 \cdot \vec{a}_1 - \frac{32}{25} \vec{S}_1 \times \vec{v}_1 \cdot \vec{a}_1 + \frac{96}{5} \log\left(\frac{r}{R_\theta}\right) \hat{n} \cdot \vec{v}_1 \hat{n} \times \vec{S}_1 \cdot \vec{v}_1 - \frac{224}{25} \hat{n} \cdot \vec{v}_1 \hat{n} \times \vec{S}_1 \cdot \vec{v}_1 \right) + \\ & \quad \frac{1}{r^4} G^3 m_1^2 m_2 \left( \frac{\frac{96}{7} (\hat{n} \cdot \vec{v}_1)^2 \hat{n} \times \vec{S}_1 \cdot \vec{v}_1 - \frac{96}{35} \vec{v}_1 \cdot \vec{v}_1 \hat{n} \times \vec{S}_1 \cdot \vec{v}_1}{\epsilon_d} - \frac{288}{7} \log\left(\frac{r}{R_\theta}\right) (\hat{n} \cdot \vec{v}_1)^2 \hat{n} \times \vec{S}_1 \cdot \vec{v}_1 + \right. \\ & \quad \left. \frac{288}{35} \log\left(\frac{r}{R_\theta}\right) \vec{v}_1 \cdot \vec{v}_1 \hat{n} \times \vec{S}_1 \cdot \vec{v}_1 + \frac{1280}{49} (\hat{n} \cdot \vec{v}_1)^2 \hat{n} \times \vec{S}_1 \cdot \vec{v}_1 - \frac{4944 \vec{v}_1 \cdot \vec{v}_1 \hat{n} \times \vec{S}_1 \cdot \vec{v}_1}{1225} \right) \Bigg\} \end{aligned}$$

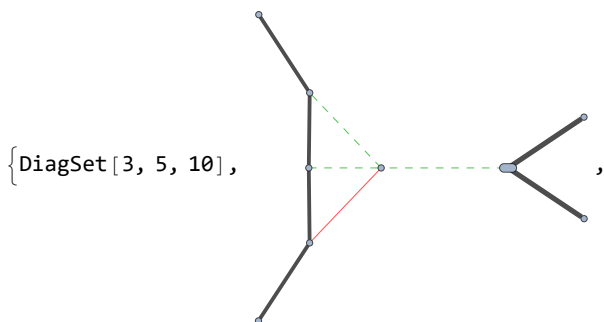

$$\begin{aligned} & \frac{1}{r^3} G^3 m_2^3 \left( \frac{32 \hat{n} \cdot \vec{a}_2 \hat{n} \times \vec{S}_1 \cdot \vec{v}_2 + 32 \hat{n} \cdot \vec{v}_2 \hat{n} \times \vec{a}_2 \cdot \vec{S}_1 - \frac{64}{3} \vec{a}_2 \times \vec{S}_1 \cdot \vec{v}_2 + 32 \hat{n} \cdot \vec{v}_2 \hat{n} \times \vec{S}_1 \cdot \vec{v}_2}{\epsilon_d} - \right. \\ & \quad 96 \log\left(\frac{r}{R_\theta}\right) \hat{n} \cdot \vec{a}_2 \hat{n} \times \vec{S}_1 \cdot \vec{v}_2 - 96 \log\left(\frac{r}{R_\theta}\right) \hat{n} \cdot \vec{v}_2 \hat{n} \times \vec{a}_2 \cdot \vec{S}_1 + 32 \hat{n} \cdot \vec{a}_2 \hat{n} \times \vec{S}_1 \cdot \vec{v}_2 + \\ & \quad \left. 32 \hat{n} \cdot \vec{v}_2 \hat{n} \times \vec{a}_2 \cdot \vec{S}_1 + 64 \log\left(\frac{r}{R_\theta}\right) \vec{a}_2 \times \vec{S}_1 \cdot \vec{v}_2 - 96 \log\left(\frac{r}{R_\theta}\right) \hat{n} \cdot \vec{v}_2 \hat{n} \times \vec{S}_1 \cdot \vec{v}_2 + 32 \hat{n} \cdot \vec{v}_2 \hat{n} \times \vec{S}_1 \cdot \vec{v}_2 \right) \Bigg\} + \end{aligned}$$



$$\frac{1}{r^4} G^3 m_2^3 \left( \frac{-32 \hat{n} \cdot \vec{v}_2 \vec{S}_1 \times \vec{v}_1 \cdot \vec{v}_2 - 160 \hat{n} \cdot \vec{v}_1 \hat{n} \cdot \vec{v}_2 \hat{n} \times \vec{S}_1 \cdot \vec{v}_2 + 32 \vec{v}_1 \cdot \vec{v}_2 \hat{n} \times \vec{S}_1 \cdot \vec{v}_2}{\epsilon_d} + \right. \\ \left. 96 \log\left(\frac{r}{R_\theta}\right) \hat{n} \cdot \vec{v}_2 \vec{S}_1 \times \vec{v}_1 \cdot \vec{v}_2 + 480 \log\left(\frac{r}{R_\theta}\right) \hat{n} \cdot \vec{v}_1 \hat{n} \cdot \vec{v}_2 \hat{n} \times \vec{S}_1 \cdot \vec{v}_2 - 96 \log\left(\frac{r}{R_\theta}\right) \vec{v}_1 \cdot \vec{v}_2 \hat{n} \times \vec{S}_1 \cdot \vec{v}_2 - \right. \\ \left. 32 \hat{n} \cdot \vec{v}_2 \vec{S}_1 \times \vec{v}_1 \cdot \vec{v}_2 - 256 \hat{n} \cdot \vec{v}_1 \hat{n} \cdot \vec{v}_2 \hat{n} \times \vec{S}_1 \cdot \vec{v}_2 + 32 \vec{v}_1 \cdot \vec{v}_2 \hat{n} \times \vec{S}_1 \cdot \vec{v}_2 + \frac{16}{5} \vec{v}_2 \cdot \vec{v}_2 \hat{n} \times \vec{S}_1 \cdot \vec{v}_2 \right) \Bigg\}$$

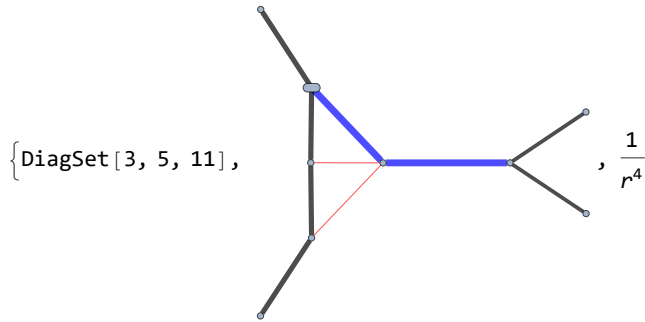

$$G^3 m_1^2 m_2 \left( \frac{1}{\epsilon_d} \left( -\frac{4}{7} (\hat{n} \cdot \vec{v}_2)^2 \hat{n} \times \vec{S}_1 \cdot \vec{v}_1 + \frac{12}{35} \hat{n} \cdot \vec{v}_2 \vec{S}_1 \times \vec{v}_1 \cdot \vec{v}_2 + \frac{4}{7} \hat{n} \cdot \vec{v}_1 \hat{n} \cdot \vec{v}_2 \hat{n} \times \vec{S}_1 \cdot \vec{v}_2 - \right. \right. \\ \left. \frac{4}{35} \vec{v}_1 \cdot \vec{v}_2 \hat{n} \times \vec{S}_1 \cdot \vec{v}_2 + \frac{4}{35} \vec{v}_2 \cdot \vec{v}_2 \hat{n} \times \vec{S}_1 \cdot \vec{v}_1 \right) + \frac{12}{7} \log\left(\frac{r}{R_\theta}\right) (\hat{n} \cdot \vec{v}_2)^2 \hat{n} \times \vec{S}_1 \cdot \vec{v}_1 - \\ \frac{36}{35} \log\left(\frac{r}{R_\theta}\right) \hat{n} \cdot \vec{v}_2 \vec{S}_1 \times \vec{v}_1 \cdot \vec{v}_2 - \frac{12}{7} \log\left(\frac{r}{R_\theta}\right) \hat{n} \cdot \vec{v}_1 \hat{n} \cdot \vec{v}_2 \hat{n} \times \vec{S}_1 \cdot \vec{v}_2 + \frac{12}{35} \log\left(\frac{r}{R_\theta}\right) \vec{v}_1 \cdot \vec{v}_2 \hat{n} \times \vec{S}_1 \cdot \vec{v}_2 - \\ \frac{12}{35} \log\left(\frac{r}{R_\theta}\right) \vec{v}_2 \cdot \vec{v}_2 \hat{n} \times \vec{S}_1 \cdot \vec{v}_1 - \frac{58}{49} (\hat{n} \cdot \vec{v}_2)^2 \hat{n} \times \vec{S}_1 \cdot \vec{v}_1 + \frac{338 \hat{n} \cdot \vec{v}_2 \vec{S}_1 \times \vec{v}_1 \cdot \vec{v}_2}{1225} + \\ \left. \frac{86}{49} \hat{n} \cdot \vec{v}_1 \hat{n} \cdot \vec{v}_2 \hat{n} \times \vec{S}_1 \cdot \vec{v}_2 - \frac{696 \vec{v}_1 \cdot \vec{v}_2 \hat{n} \times \vec{S}_1 \cdot \vec{v}_2}{1225} + \frac{556 \vec{v}_2 \cdot \vec{v}_2 \hat{n} \times \vec{S}_1 \cdot \vec{v}_1}{1225} \right) \Bigg\}$$

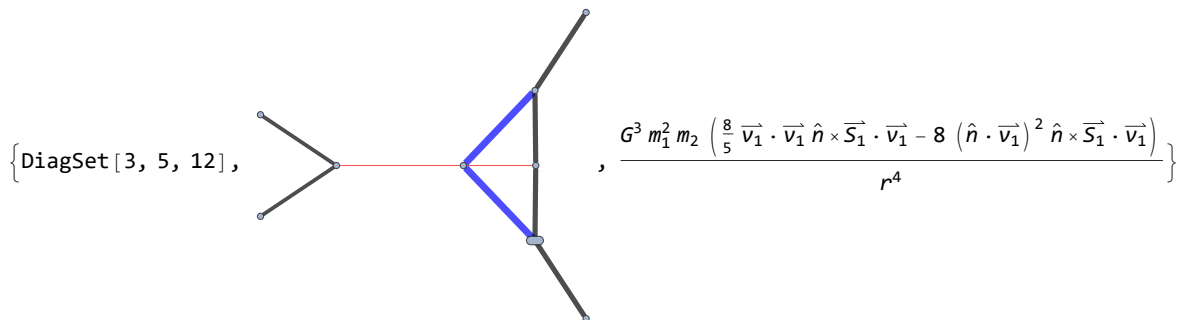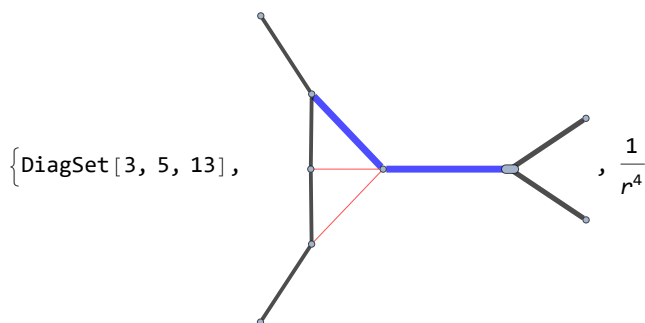

$$G^3 m_2^3 \left( \frac{1}{\epsilon_d} \left( -4 (\hat{n} \cdot \vec{v}_2)^2 \hat{n} \times \vec{S}_1 \cdot \vec{v}_1 + \frac{12}{5} \hat{n} \cdot \vec{v}_2 \vec{S}_1 \times \vec{v}_1 \cdot \vec{v}_2 + 4 \hat{n} \cdot \vec{v}_1 \hat{n} \cdot \vec{v}_2 \hat{n} \times \vec{S}_1 \cdot \vec{v}_2 - \frac{4}{5} \vec{v}_1 \cdot \vec{v}_2 \hat{n} \times \vec{S}_1 \cdot \vec{v}_2 + \right. \right.$$

$$\begin{aligned} & \frac{4}{5} \vec{v}_2 \cdot \vec{v}_2 \hat{n} \times \vec{S}_1 \cdot \vec{v}_1 \Big) + 12 \log \left( \frac{r}{R_\theta} \right) (\hat{n} \cdot \vec{v}_2)^2 \hat{n} \times \vec{S}_1 \cdot \vec{v}_1 - \frac{36}{5} \log \left( \frac{r}{R_\theta} \right) \hat{n} \cdot \vec{v}_2 \vec{S}_1 \times \vec{v}_1 \cdot \vec{v}_2 - \\ & 12 \log \left( \frac{r}{R_\theta} \right) \hat{n} \cdot \vec{v}_1 \hat{n} \cdot \vec{v}_2 \hat{n} \times \vec{S}_1 \cdot \vec{v}_2 + \frac{12}{5} \log \left( \frac{r}{R_\theta} \right) \vec{v}_1 \cdot \vec{v}_2 \hat{n} \times \vec{S}_1 \cdot \vec{v}_2 - \frac{12}{5} \log \left( \frac{r}{R_\theta} \right) \vec{v}_2 \cdot \vec{v}_2 \hat{n} \times \vec{S}_1 \cdot \vec{v}_1 - \\ & 6 \left( \hat{n} \cdot \vec{v}_2 \right)^2 \hat{n} \times \vec{S}_1 \cdot \vec{v}_1 + \frac{74}{25} \hat{n} \cdot \vec{v}_2 \vec{S}_1 \times \vec{v}_1 \cdot \vec{v}_2 + 10 \hat{n} \cdot \vec{v}_1 \hat{n} \cdot \vec{v}_2 \hat{n} \times \vec{S}_1 \cdot \vec{v}_2 - \frac{48}{25} \vec{v}_1 \cdot \vec{v}_2 \hat{n} \times \vec{S}_1 \cdot \vec{v}_2 + \frac{28}{25} \vec{v}_2 \cdot \vec{v}_2 \hat{n} \times \vec{S}_1 \cdot \vec{v}_1 \Big) \} \end{aligned}$$

$\{\text{DiagSet}[3, 5, 14],$

$, \frac{1}{r^4}$

$$\begin{aligned} & G^3 m_1^2 m_2 \left( \frac{-\frac{4}{7} (\hat{n} \cdot \vec{v}_1)^2 \hat{n} \times \vec{S}_1 \cdot \vec{v}_2 - \frac{8}{35} \hat{n} \cdot \vec{v}_1 \vec{S}_1 \times \vec{v}_1 \cdot \vec{v}_2 + \frac{4}{35} \vec{v}_1 \cdot \vec{v}_1 \hat{n} \times \vec{S}_1 \cdot \vec{v}_2}{\epsilon_d} + \right. \\ & \frac{12}{7} \log \left( \frac{r}{R_\theta} \right) (\hat{n} \cdot \vec{v}_1)^2 \hat{n} \times \vec{S}_1 \cdot \vec{v}_2 + \frac{24}{35} \log \left( \frac{r}{R_\theta} \right) \hat{n} \cdot \vec{v}_1 \vec{S}_1 \times \vec{v}_1 \cdot \vec{v}_2 - \frac{12}{35} \log \left( \frac{r}{R_\theta} \right) \vec{v}_1 \cdot \vec{v}_1 \hat{n} \times \vec{S}_1 \cdot \vec{v}_2 - \\ & \left. \frac{86}{49} (\hat{n} \cdot \vec{v}_1)^2 \hat{n} \times \vec{S}_1 \cdot \vec{v}_2 - \frac{412 \hat{n} \cdot \vec{v}_1 \vec{S}_1 \times \vec{v}_1 \cdot \vec{v}_2}{1225} + \frac{206 \vec{v}_1 \cdot \vec{v}_1 \hat{n} \times \vec{S}_1 \cdot \vec{v}_2}{1225} \right) \} \end{aligned}$$

$\{\text{DiagSet}[3, 5, 15],$

$, \frac{1}{r^4} G^3 m_1^2 m_2$

$$\begin{aligned} & \left( \frac{1}{\epsilon_d} \left( 4 (\hat{n} \cdot \vec{v}_1)^2 \hat{n} \times \vec{S}_1 \cdot \vec{v}_1 - \frac{4}{5} \hat{n} \cdot \vec{v}_1 \vec{S}_1 \times \vec{v}_1 \cdot \vec{v}_2 + 4 \hat{n} \cdot \vec{v}_2 \hat{n} \cdot \vec{v}_1 \hat{n} \times \vec{S}_1 \cdot \vec{v}_1 - \frac{4}{5} \vec{v}_1 \cdot \vec{v}_1 \hat{n} \times \vec{S}_1 \cdot \vec{v}_1 - \frac{4}{5} \vec{v}_1 \cdot \vec{v}_2 \hat{n} \times \vec{S}_1 \cdot \vec{v}_1 \right) - \right. \\ & 12 \log \left( \frac{r}{R_\theta} \right) (\hat{n} \cdot \vec{v}_1)^2 \hat{n} \times \vec{S}_1 \cdot \vec{v}_1 + \frac{12}{5} \log \left( \frac{r}{R_\theta} \right) \hat{n} \cdot \vec{v}_1 \vec{S}_1 \times \vec{v}_1 \cdot \vec{v}_2 - 12 \log \left( \frac{r}{R_\theta} \right) \hat{n} \cdot \vec{v}_2 \hat{n} \cdot \vec{v}_1 \hat{n} \times \vec{S}_1 \cdot \vec{v}_1 + \\ & \frac{12}{5} \log \left( \frac{r}{R_\theta} \right) \vec{v}_1 \cdot \vec{v}_1 \hat{n} \times \vec{S}_1 \cdot \vec{v}_1 + \frac{12}{5} \log \left( \frac{r}{R_\theta} \right) \vec{v}_1 \cdot \vec{v}_2 \hat{n} \times \vec{S}_1 \cdot \vec{v}_1 + 10 (\hat{n} \cdot \vec{v}_1)^2 \hat{n} \times \vec{S}_1 \cdot \vec{v}_1 - \\ & \left. \frac{38}{25} \hat{n} \cdot \vec{v}_1 \vec{S}_1 \times \vec{v}_1 \cdot \vec{v}_2 + 10 \hat{n} \cdot \vec{v}_2 \hat{n} \cdot \vec{v}_1 \hat{n} \times \vec{S}_1 \cdot \vec{v}_1 - \frac{58}{25} \vec{v}_1 \cdot \vec{v}_1 \hat{n} \times \vec{S}_1 \cdot \vec{v}_1 - \frac{38}{25} \vec{v}_1 \cdot \vec{v}_2 \hat{n} \times \vec{S}_1 \cdot \vec{v}_1 \right) \} \end{aligned}$$

$\{\text{DiagSet}[3, 5, 16],$

$, \frac{1}{r^4}$

$$G^3 m_1^2 m_2 \left( \frac{-\frac{4}{35} \hat{n} \cdot \vec{v}_2 \vec{S}_1 \times \vec{v}_1 \cdot \vec{v}_2 - \frac{4}{7} \hat{n} \cdot \vec{v}_1 \hat{n} \cdot \vec{v}_2 \hat{n} \times \vec{S}_1 \cdot \vec{v}_2 + \frac{4}{35} \vec{v}_1 \cdot \vec{v}_2 \hat{n} \times \vec{S}_1 \cdot \vec{v}_2}{\epsilon_d} + \right. \\ \left. \frac{12}{35} \log\left(\frac{r}{R_\theta}\right) \hat{n} \cdot \vec{v}_2 \vec{S}_1 \times \vec{v}_1 \cdot \vec{v}_2 + \frac{12}{7} \log\left(\frac{r}{R_\theta}\right) \hat{n} \cdot \vec{v}_1 \hat{n} \cdot \vec{v}_2 \hat{n} \times \vec{S}_1 \cdot \vec{v}_2 - \frac{12}{35} \log\left(\frac{r}{R_\theta}\right) \vec{v}_1 \cdot \vec{v}_2 \hat{n} \times \vec{S}_1 \cdot \vec{v}_2 - \right. \\ \left. \frac{206 \hat{n} \cdot \vec{v}_2 \vec{S}_1 \times \vec{v}_1 \cdot \vec{v}_2}{1225} - \frac{86}{49} \hat{n} \cdot \vec{v}_1 \hat{n} \cdot \vec{v}_2 \hat{n} \times \vec{S}_1 \cdot \vec{v}_2 + \frac{206 \vec{v}_1 \cdot \vec{v}_2 \hat{n} \times \vec{S}_1 \cdot \vec{v}_2}{1225} \right\}$$

{DiagSet[3, 5, 17], 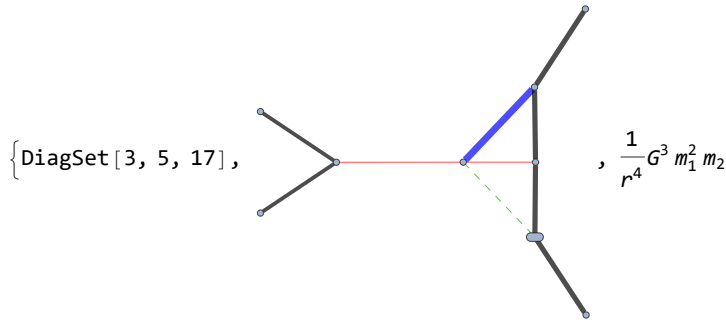 ,  $\frac{1}{r^4} G^3 m_1^2 m_2$

$$\left( \frac{1}{\epsilon_d} \left( 4 (\hat{n} \cdot \vec{v}_1)^2 \hat{n} \times \vec{S}_1 \cdot \vec{v}_1 - \frac{4}{5} \hat{n} \cdot \vec{v}_1 \vec{S}_1 \times \vec{v}_1 \cdot \vec{v}_2 + 4 \hat{n} \cdot \vec{v}_2 \hat{n} \cdot \vec{v}_1 \hat{n} \times \vec{S}_1 \cdot \vec{v}_1 - \frac{4}{5} \vec{v}_1 \cdot \vec{v}_1 \hat{n} \times \vec{S}_1 \cdot \vec{v}_1 - \frac{4}{5} \vec{v}_1 \cdot \vec{v}_2 \hat{n} \times \vec{S}_1 \cdot \vec{v}_1 \right) - \right. \\ \left. 12 \log\left(\frac{r}{R_\theta}\right) (\hat{n} \cdot \vec{v}_1)^2 \hat{n} \times \vec{S}_1 \cdot \vec{v}_1 + \frac{12}{5} \log\left(\frac{r}{R_\theta}\right) \hat{n} \cdot \vec{v}_1 \vec{S}_1 \times \vec{v}_1 \cdot \vec{v}_2 - 12 \log\left(\frac{r}{R_\theta}\right) \hat{n} \cdot \vec{v}_2 \hat{n} \cdot \vec{v}_1 \hat{n} \times \vec{S}_1 \cdot \vec{v}_1 + \right. \\ \left. \frac{12}{5} \log\left(\frac{r}{R_\theta}\right) \vec{v}_1 \cdot \vec{v}_1 \hat{n} \times \vec{S}_1 \cdot \vec{v}_1 + \frac{12}{5} \log\left(\frac{r}{R_\theta}\right) \vec{v}_1 \cdot \vec{v}_2 \hat{n} \times \vec{S}_1 \cdot \vec{v}_1 + 10 (\hat{n} \cdot \vec{v}_1)^2 \hat{n} \times \vec{S}_1 \cdot \vec{v}_1 - \right. \\ \left. \frac{38}{25} \hat{n} \cdot \vec{v}_1 \vec{S}_1 \times \vec{v}_1 \cdot \vec{v}_2 + 10 \hat{n} \cdot \vec{v}_2 \hat{n} \cdot \vec{v}_1 \hat{n} \times \vec{S}_1 \cdot \vec{v}_1 - \frac{38}{25} \vec{v}_1 \cdot \vec{v}_1 \hat{n} \times \vec{S}_1 \cdot \vec{v}_1 - \frac{38}{25} \vec{v}_1 \cdot \vec{v}_2 \hat{n} \times \vec{S}_1 \cdot \vec{v}_1 \right) \}$$

{DiagSet[3, 5, 18], 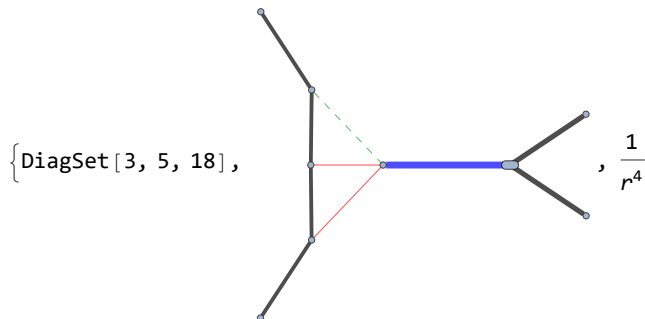 ,  $\frac{1}{r^4}$

$$G^3 m_2^3 \left( \frac{-\frac{4}{5} \hat{n} \cdot \vec{v}_2 \vec{S}_1 \times \vec{v}_1 \cdot \vec{v}_2 - 4 \hat{n} \cdot \vec{v}_1 \hat{n} \cdot \vec{v}_2 \hat{n} \times \vec{S}_1 \cdot \vec{v}_2 + \frac{4}{5} \vec{v}_1 \cdot \vec{v}_2 \hat{n} \times \vec{S}_1 \cdot \vec{v}_2}{\epsilon_d} + \right. \\ \left. \frac{12}{5} \log\left(\frac{r}{R_\theta}\right) \hat{n} \cdot \vec{v}_2 \vec{S}_1 \times \vec{v}_1 \cdot \vec{v}_2 + 12 \log\left(\frac{r}{R_\theta}\right) \hat{n} \cdot \vec{v}_1 \hat{n} \cdot \vec{v}_2 \hat{n} \times \vec{S}_1 \cdot \vec{v}_2 - \frac{12}{5} \log\left(\frac{r}{R_\theta}\right) \vec{v}_1 \cdot \vec{v}_2 \hat{n} \times \vec{S}_1 \cdot \vec{v}_2 - \right. \\ \left. \frac{38}{25} \hat{n} \cdot \vec{v}_2 \vec{S}_1 \times \vec{v}_1 \cdot \vec{v}_2 - 10 \hat{n} \cdot \vec{v}_1 \hat{n} \cdot \vec{v}_2 \hat{n} \times \vec{S}_1 \cdot \vec{v}_2 - \frac{2}{25} \vec{v}_1 \cdot \vec{v}_2 \hat{n} \times \vec{S}_1 \cdot \vec{v}_2 \right\}$$

$\{\text{DiagSet}[3, 5, 19],$ 
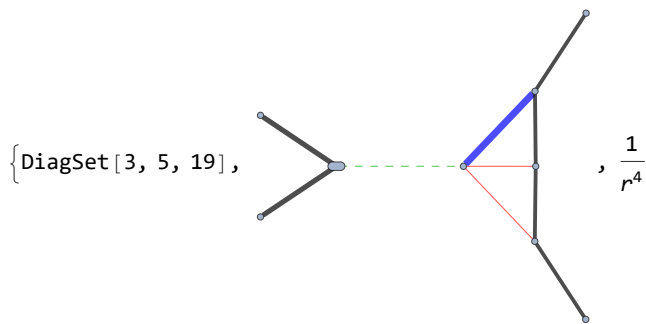
 $, \frac{1}{r^4}$

$$G^3 m_2^3 \left( \frac{\frac{4}{5} \vec{v}_2 \cdot \vec{v}_2 \hat{n} \times \vec{S}_1 \cdot \vec{v}_2 - 4 (\hat{n} \cdot \vec{v}_2)^2 \hat{n} \times \vec{S}_1 \cdot \vec{v}_2}{\epsilon_d} + 12 \log\left(\frac{r}{R_\theta}\right) (\hat{n} \cdot \vec{v}_2)^2 \hat{n} \times \vec{S}_1 \cdot \vec{v}_2 - \right.$$

$$\left. \frac{12}{5} \log\left(\frac{r}{R_\theta}\right) \vec{v}_2 \cdot \vec{v}_2 \hat{n} \times \vec{S}_1 \cdot \vec{v}_2 - 10 (\hat{n} \cdot \vec{v}_2)^2 \hat{n} \times \vec{S}_1 \cdot \vec{v}_2 + \frac{18}{25} \vec{v}_2 \cdot \vec{v}_2 \hat{n} \times \vec{S}_1 \cdot \vec{v}_2 \right\}$$

$\{\text{DiagSet}[3, 5, 20],$ 
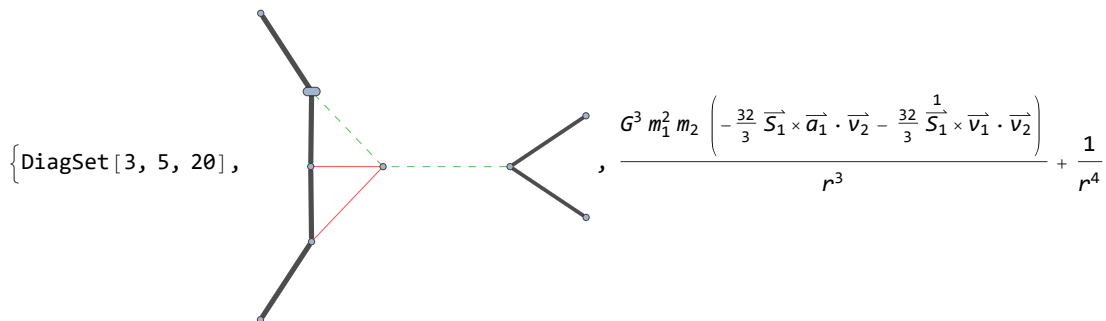
 $, \frac{G^3 m_1^2 m_2 \left( -\frac{32}{3} \vec{S}_1 \times \vec{a}_1 \cdot \vec{v}_2 - \frac{32}{3} \vec{S}_1 \times \vec{v}_1 \cdot \vec{v}_2 \right)}{r^3} + \frac{1}{r^4}$

$$G^3 m_1^2 m_2 \left( \frac{\frac{4}{7} (\hat{n} \cdot \vec{v}_1)^2 \hat{n} \times \vec{S}_1 \cdot \vec{v}_2 + \frac{8}{35} \hat{n} \cdot \vec{v}_1 \vec{S}_1 \times \vec{v}_1 \cdot \vec{v}_2 - \frac{4}{35} \vec{v}_1 \cdot \vec{v}_1 \hat{n} \times \vec{S}_1 \cdot \vec{v}_2}{\epsilon_d} - \frac{12}{7} \log\left(\frac{r}{R_\theta}\right) (\hat{n} \cdot \vec{v}_1)^2 \hat{n} \times \vec{S}_1 \cdot \vec{v}_2 - \right.$$

$$\frac{24}{35} \log\left(\frac{r}{R_\theta}\right) \hat{n} \cdot \vec{v}_1 \vec{S}_1 \times \vec{v}_1 \cdot \vec{v}_2 + \frac{12}{35} \log\left(\frac{r}{R_\theta}\right) \vec{v}_1 \cdot \vec{v}_1 \hat{n} \times \vec{S}_1 \cdot \vec{v}_2 + \frac{86}{49} (\hat{n} \cdot \vec{v}_1)^2 \hat{n} \times \vec{S}_1 \cdot \vec{v}_2 +$$

$$\left. \frac{10212 \hat{n} \cdot \vec{v}_1 \vec{S}_1 \times \vec{v}_1 \cdot \vec{v}_2}{1225} + \frac{11554 \vec{v}_1 \cdot \vec{v}_1 \hat{n} \times \vec{S}_1 \cdot \vec{v}_2}{1225} + \frac{56}{5} \vec{v}_1 \cdot \vec{v}_2 \hat{n} \times \vec{S}_1 \cdot \vec{v}_1 + \frac{8}{5} \vec{v}_2 \cdot \vec{v}_2 \hat{n} \times \vec{S}_1 \cdot \vec{v}_2 \right\}$$

$\{\text{DiagSet}[3, 5, 21],$ 
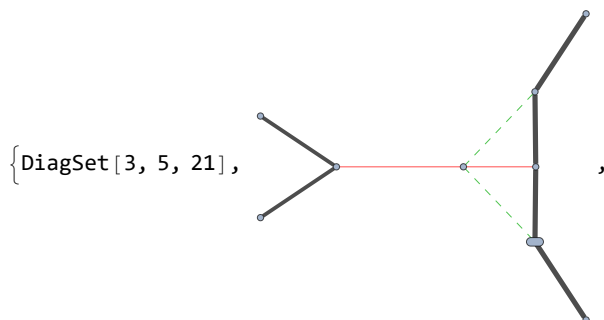
 $,$

$$\frac{1}{r^4} G^3 m_1^2 m_2 \left( \frac{\frac{8}{5} \hat{n} \cdot \vec{v}_1 \vec{S}_1 \times \vec{v}_1 \cdot \vec{v}_2 - 8 \hat{n} \cdot \vec{v}_2 \hat{n} \cdot \vec{v}_1 \hat{n} \times \vec{S}_1 \cdot \vec{v}_1 + \frac{8}{5} \vec{v}_1 \cdot \vec{v}_2 \hat{n} \times \vec{S}_1 \cdot \vec{v}_1}{\epsilon_d} - \frac{24}{5} \log\left(\frac{r}{R_\theta}\right) \hat{n} \cdot \vec{v}_1 \vec{S}_1 \times \vec{v}_1 \cdot \vec{v}_2 + \right.$$

$$\left. 24 \log\left(\frac{r}{R_\theta}\right) \hat{n} \cdot \vec{v}_2 \hat{n} \cdot \vec{v}_1 \hat{n} \times \vec{S}_1 \cdot \vec{v}_1 - \frac{24}{5} \log\left(\frac{r}{R_\theta}\right) \vec{v}_1 \cdot \vec{v}_2 \hat{n} \times \vec{S}_1 \cdot \vec{v}_1 + \frac{76}{25} \hat{n} \cdot \vec{v}_1 \vec{S}_1 \times \vec{v}_1 \cdot \vec{v}_2 - 20 \hat{n} \cdot \vec{v}_2 \hat{n} \cdot \vec{v}_1 \right.$$

$$\hat{n} \times \vec{S}_1 \cdot \vec{v}_1 - \frac{88}{5} \vec{v}_1 \cdot \vec{v}_1 \hat{n} \times \vec{S}_1 \cdot \vec{v}_1 + \frac{76}{25} \vec{v}_1 \cdot \vec{v}_2 \hat{n} \times \vec{S}_1 \cdot \vec{v}_1 - \frac{24}{5} \vec{v}_2 \cdot \vec{v}_2 \hat{n} \times \vec{S}_1 \cdot \vec{v}_1 \left\} - \frac{32 G^3 m_1^2 m_2 \vec{S}_1 \times \vec{v}_1 \cdot \vec{a}_1}{3 r^3} \right\}$$

{DiagSet[3, 5, 22], 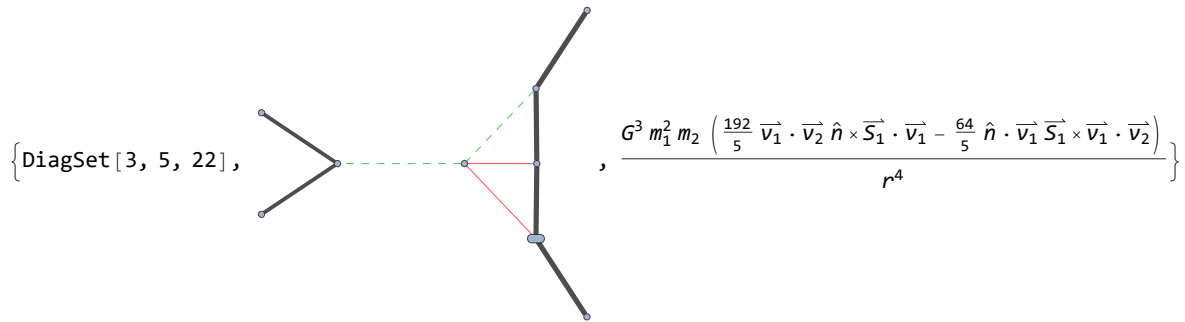 , 
$$\frac{G^3 m_1^2 m_2 \left( \frac{192}{5} \vec{v}_1 \cdot \vec{v}_2 \hat{n} \times \vec{S}_1 \cdot \vec{v}_1 - \frac{64}{5} \hat{n} \cdot \vec{v}_1 \vec{S}_1 \times \vec{v}_1 \cdot \vec{v}_2 \right)}{r^4}$$
 }

{DiagSet[3, 5, 23], 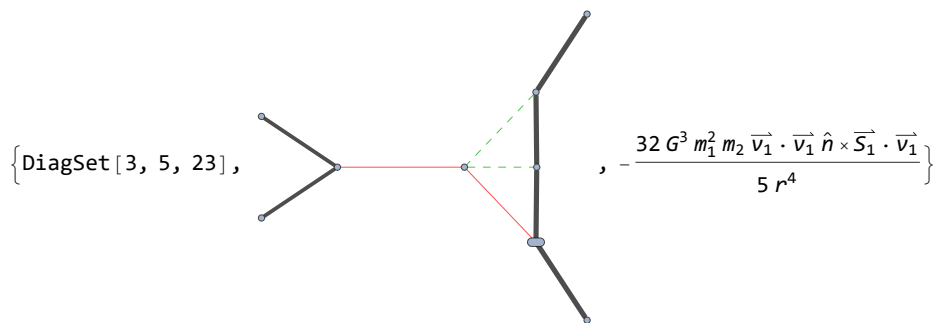 , 
$$-\frac{32 G^3 m_1^2 m_2 \vec{v}_1 \cdot \vec{v}_1 \hat{n} \times \vec{S}_1 \cdot \vec{v}_1}{5 r^4}$$
 }

{DiagSet[3, 5, 24], 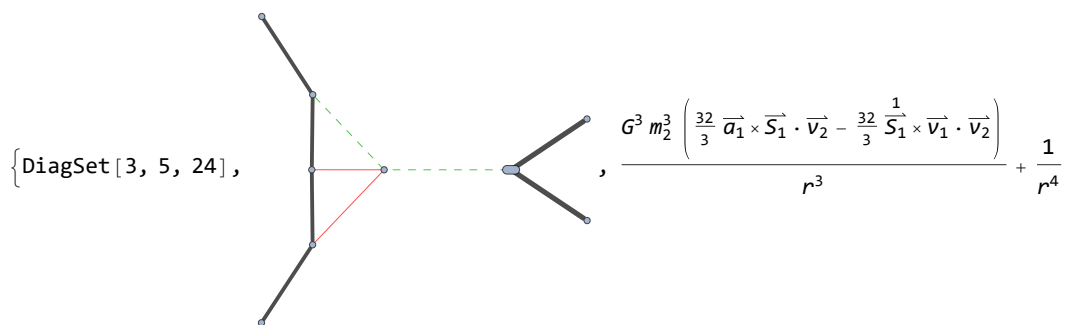 , 
$$\frac{G^3 m_2^3 \left( \frac{32}{3} \vec{a}_1 \times \vec{S}_1 \cdot \vec{v}_2 - \frac{32}{3} \vec{S}_1 \times \vec{v}_1 \cdot \vec{v}_2 \right)}{r^3} + \frac{1}{r^4}$$
 }

$$G^3 m_2^3 \left\{ \frac{4 (\hat{n} \cdot \vec{v}_2)^2 \hat{n} \times \vec{S}_1 \cdot \vec{v}_2 - \frac{4}{5} \vec{v}_2 \cdot \vec{v}_2 \hat{n} \times \vec{S}_1 \cdot \vec{v}_2}{\epsilon_d} - 12 \log \left( \frac{r}{R_0} \right) (\hat{n} \cdot \vec{v}_2)^2 \hat{n} \times \vec{S}_1 \cdot \vec{v}_2 + \frac{12}{5} \log \left( \frac{r}{R_0} \right) \vec{v}_2 \cdot \vec{v}_2 \hat{n} \times \vec{S}_1 \cdot \vec{v}_2 + \right. \\ \left. 10 (\hat{n} \cdot \vec{v}_2)^2 \hat{n} \times \vec{S}_1 \cdot \vec{v}_2 + 8 \hat{n} \cdot \vec{v}_1 \vec{S}_1 \times \vec{v}_1 \cdot \vec{v}_2 + 24 \vec{v}_1 \cdot \vec{v}_2 \hat{n} \times \vec{S}_1 \cdot \vec{v}_1 + \frac{1382}{25} \vec{v}_2 \cdot \vec{v}_2 \hat{n} \times \vec{S}_1 \cdot \vec{v}_2 \right\}$$

{DiagSet[3, 5, 25], 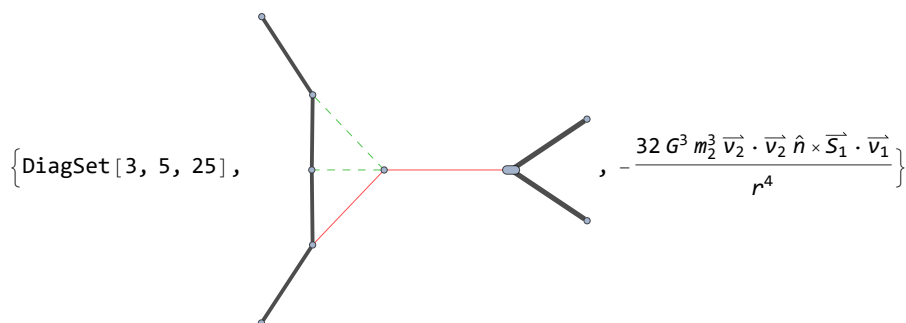 , 
$$-\frac{32 G^3 m_2^3 \vec{v}_2 \cdot \vec{v}_2 \hat{n} \times \vec{S}_1 \cdot \vec{v}_1}{r^4}$$
 }

$\{\text{DiagSet}[3, 5, 26],$ 
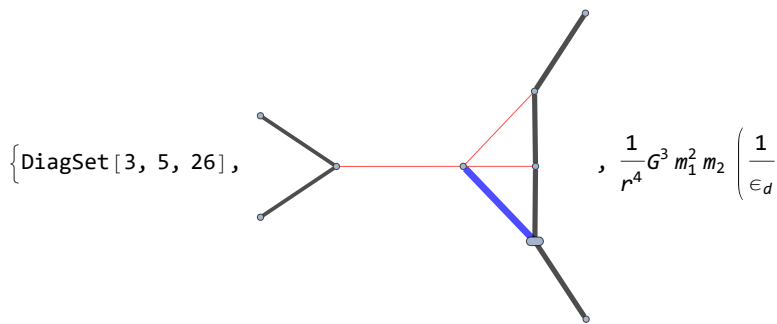
 $, \frac{1}{r^4} G^3 m_1^2 m_2 \left( \frac{1}{\epsilon_d} \right.$

$$\begin{aligned}
 & \left( \frac{4}{7} (\hat{n} \cdot \vec{v}_1)^2 \hat{n} \times \vec{S}_1 \cdot \vec{v}_1 + \frac{8}{5} \hat{n} \cdot \vec{v}_1 \vec{S}_1 \times \vec{v}_1 \cdot \vec{v}_2 - 8 \hat{n} \cdot \vec{v}_2 \hat{n} \cdot \vec{v}_1 \hat{n} \times \vec{S}_1 \cdot \vec{v}_1 - \frac{4}{35} \vec{v}_1 \cdot \vec{v}_1 \hat{n} \times \vec{S}_1 \cdot \vec{v}_1 + \frac{8}{5} \vec{v}_1 \cdot \vec{v}_2 \hat{n} \times \vec{S}_1 \cdot \vec{v}_1 \right) - \\
 & \frac{12}{7} \log\left(\frac{r}{R_\theta}\right) (\hat{n} \cdot \vec{v}_1)^2 \hat{n} \times \vec{S}_1 \cdot \vec{v}_1 - \frac{24}{5} \log\left(\frac{r}{R_\theta}\right) \hat{n} \cdot \vec{v}_1 \vec{S}_1 \times \vec{v}_1 \cdot \vec{v}_2 + 24 \log\left(\frac{r}{R_\theta}\right) \hat{n} \cdot \vec{v}_2 \hat{n} \cdot \vec{v}_1 \hat{n} \times \vec{S}_1 \cdot \vec{v}_1 + \\
 & \frac{12}{35} \log\left(\frac{r}{R_\theta}\right) \vec{v}_1 \cdot \vec{v}_1 \hat{n} \times \vec{S}_1 \cdot \vec{v}_1 - \frac{24}{5} \log\left(\frac{r}{R_\theta}\right) \vec{v}_1 \cdot \vec{v}_2 \hat{n} \times \vec{S}_1 \cdot \vec{v}_1 + \frac{58}{49} (\hat{n} \cdot \vec{v}_1)^2 \hat{n} \times \vec{S}_1 \cdot \vec{v}_1 + \\
 & \left. \frac{36}{25} \hat{n} \cdot \vec{v}_1 \vec{S}_1 \times \vec{v}_1 \cdot \vec{v}_2 - 12 \hat{n} \cdot \vec{v}_2 \hat{n} \cdot \vec{v}_1 \hat{n} \times \vec{S}_1 \cdot \vec{v}_1 - \frac{66 \vec{v}_1 \cdot \vec{v}_1 \hat{n} \times \vec{S}_1 \cdot \vec{v}_1}{1225} + \frac{36}{25} \vec{v}_1 \cdot \vec{v}_2 \hat{n} \times \vec{S}_1 \cdot \vec{v}_1 \right\}
 \end{aligned}$$

$\{\text{DiagSet}[3, 5, 27],$ 
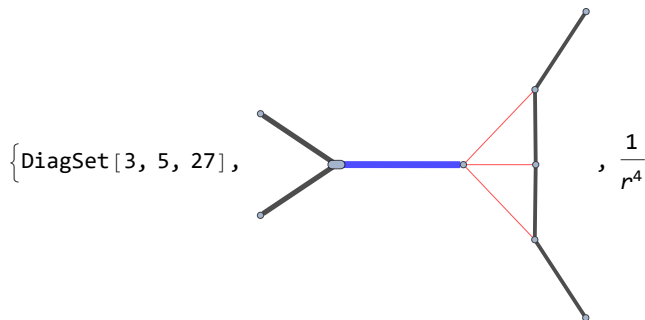
 $, \frac{1}{r^4}$

$$\begin{aligned}
 & G^3 m_2^3 \left( \frac{4 (\hat{n} \cdot \vec{v}_2)^2 \hat{n} \times \vec{S}_1 \cdot \vec{v}_1 - \frac{8}{5} \hat{n} \cdot \vec{v}_2 \vec{S}_1 \times \vec{v}_1 \cdot \vec{v}_2 - \frac{4}{5} \vec{v}_2 \cdot \vec{v}_2 \hat{n} \times \vec{S}_1 \cdot \vec{v}_1}{\epsilon_d} - \right. \\
 & 12 \log\left(\frac{r}{R_\theta}\right) (\hat{n} \cdot \vec{v}_2)^2 \hat{n} \times \vec{S}_1 \cdot \vec{v}_1 + \frac{24}{5} \log\left(\frac{r}{R_\theta}\right) \hat{n} \cdot \vec{v}_2 \vec{S}_1 \times \vec{v}_1 \cdot \vec{v}_2 + \frac{12}{5} \log\left(\frac{r}{R_\theta}\right) \vec{v}_2 \cdot \vec{v}_2 \hat{n} \times \vec{S}_1 \cdot \vec{v}_1 + \\
 & \left. 6 (\hat{n} \cdot \vec{v}_2)^2 \hat{n} \times \vec{S}_1 \cdot \vec{v}_1 - \frac{36}{25} \hat{n} \cdot \vec{v}_2 \vec{S}_1 \times \vec{v}_1 \cdot \vec{v}_2 + \frac{2}{25} \vec{v}_2 \cdot \vec{v}_2 \hat{n} \times \vec{S}_1 \cdot \vec{v}_1 \right\}
 \end{aligned}$$

$\{\text{DiagSet}[3, 5, 28],$ 
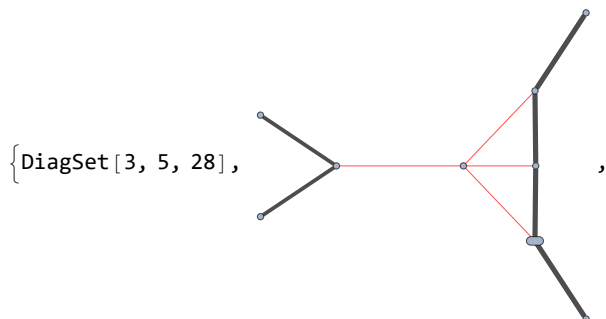
 $,$

$$\begin{aligned}
 & \frac{1}{r^3} m_1^2 m_2 \left( -\frac{16}{5} \log\left(\frac{r}{R_\theta}\right) \vec{S}_1 \times \vec{v}_1 \cdot \vec{a}_1 - \frac{16}{25} \vec{S}_1 \times \vec{v}_1 \cdot \vec{a}_1 + \frac{112}{25} \hat{n} \times \vec{S}_1 \cdot \vec{v}_1 \hat{n} \cdot \vec{v}_1 + \frac{112}{25} \hat{n} \times \vec{S}_1 \cdot \vec{a}_1 \hat{n} \cdot \vec{v}_1 - \right. \\
 & \left. 8 \hat{n} \times \vec{S}_1 \cdot \vec{v}_1 \hat{n} \cdot \vec{v}_2 - 8 \hat{n} \times \vec{S}_1 \cdot \vec{a}_1 \hat{n} \cdot \vec{v}_2 - 8 \vec{S}_1 \times \vec{v}_1 \cdot \vec{v}_2 \log\left(\frac{r}{R_\theta}\right) - 8 \vec{S}_1 \times \vec{a}_1 \cdot \vec{v}_2 \log\left(\frac{r}{R_\theta}\right) - \right.
 \end{aligned}$$

$$\begin{aligned} & \frac{48}{5} \hat{n} \times \vec{S}_1 \cdot \vec{v}_1 \hat{n} \cdot \vec{v}_1 \log\left(\frac{r}{R_\theta}\right) - \frac{48}{5} \hat{n} \times \vec{S}_1 \cdot \vec{a}_1 \hat{n} \cdot \vec{v}_1 \log\left(\frac{r}{R_\theta}\right) + 24 \hat{n} \times \vec{S}_1 \cdot \vec{v}_1 \hat{n} \cdot \vec{v}_2 \log\left(\frac{r}{R_\theta}\right) + \\ & 24 \hat{n} \times \vec{S}_1 \cdot \vec{a}_1 \hat{n} \cdot \vec{v}_2 \log\left(\frac{r}{R_\theta}\right) + \frac{1}{\epsilon_d} \left( \frac{8}{3} \vec{S}_1 \times \vec{v}_1 \cdot \vec{v}_2 + \frac{8}{3} \vec{S}_1 \times \vec{a}_1 \cdot \vec{v}_2 + \frac{16}{15} \vec{S}_1 \times \vec{v}_1 \cdot \vec{a}_1 + \right. \\ & \left. \frac{16}{5} \hat{n} \times \vec{S}_1 \cdot \vec{v}_1 \hat{n} \cdot \vec{v}_1 + \frac{16}{5} \hat{n} \times \vec{S}_1 \cdot \vec{a}_1 \hat{n} \cdot \vec{v}_1 - 8 \hat{n} \times \vec{S}_1 \cdot \vec{v}_1 \hat{n} \cdot \vec{v}_2 - 8 \hat{n} \times \vec{S}_1 \cdot \vec{a}_1 \hat{n} \cdot \vec{v}_2 \right) \Bigg) G^3 + \frac{1}{r^4} \\ & m_1^2 m_2 \left( -16 \hat{n} \times \vec{S}_1 \cdot \vec{v}_1 (\hat{n} \cdot \vec{v}_1)^2 + 24 \hat{n} \times \vec{S}_1 \cdot \vec{v}_1 \log\left(\frac{r}{R_\theta}\right) (\hat{n} \cdot \vec{v}_1)^2 - 8 \vec{S}_1 \times \vec{v}_1 \cdot \vec{v}_2 \hat{n} \cdot \vec{v}_1 + 64 \hat{n} \times \vec{S}_1 \cdot \vec{v}_1 \hat{n} \cdot \vec{v}_2 \hat{n} \cdot \vec{v}_1 + \right. \\ & 24 \vec{S}_1 \times \vec{v}_1 \cdot \vec{v}_2 \log\left(\frac{r}{R_\theta}\right) \hat{n} \cdot \vec{v}_1 - 120 \hat{n} \times \vec{S}_1 \cdot \vec{v}_1 \hat{n} \cdot \vec{v}_2 \log\left(\frac{r}{R_\theta}\right) \hat{n} \cdot \vec{v}_1 + \frac{16}{25} \hat{n} \times \vec{S}_1 \cdot \vec{v}_1 \vec{v}_1 \cdot \vec{v}_1 - 8 \hat{n} \times \vec{S}_1 \cdot \vec{v}_1 \vec{v}_1 \cdot \vec{v}_2 - \\ & \left. \frac{24}{5} \hat{n} \times \vec{S}_1 \cdot \vec{v}_1 \vec{v}_1 \cdot \vec{v}_1 \log\left(\frac{r}{R_\theta}\right) + 24 \hat{n} \times \vec{S}_1 \cdot \vec{v}_1 \vec{v}_1 \cdot \vec{v}_2 \log\left(\frac{r}{R_\theta}\right) + \frac{1}{\epsilon_d} \left( -8 \hat{n} \times \vec{S}_1 \cdot \vec{v}_1 (\hat{n} \cdot \vec{v}_1)^2 - \right. \right. \\ & \left. \left. 8 \vec{S}_1 \times \vec{v}_1 \cdot \vec{v}_2 \hat{n} \cdot \vec{v}_1 + 40 \hat{n} \times \vec{S}_1 \cdot \vec{v}_1 \hat{n} \cdot \vec{v}_2 \hat{n} \cdot \vec{v}_1 + \frac{8}{5} \hat{n} \times \vec{S}_1 \cdot \vec{v}_1 \vec{v}_1 \cdot \vec{v}_1 - 8 \hat{n} \times \vec{S}_1 \cdot \vec{v}_1 \vec{v}_1 \cdot \vec{v}_2 \right) \right) G^3 \Bigg\} \end{aligned}$$

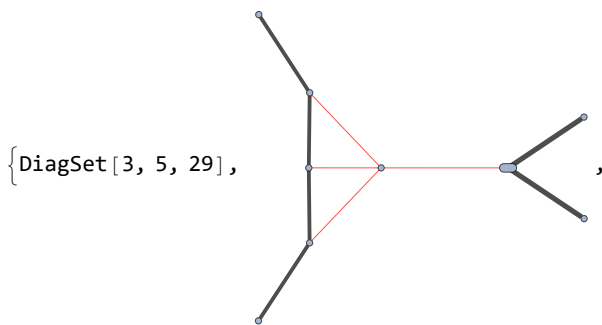

$$\begin{aligned} & \frac{1}{r^3} G^3 m_2^3 \left( \frac{8 \hat{n} \cdot \vec{v}_2 \hat{n} \cdot \vec{a}_1 \cdot \vec{S}_1 - \frac{8}{3} \vec{a}_1 \times \vec{S}_1 \cdot \vec{v}_2 - 8 \hat{n} \cdot \vec{v}_2 \hat{n} \times \vec{S}_1 \cdot \vec{v}_1 + \frac{8}{3} \vec{S}_1 \times \vec{v}_1 \cdot \vec{v}_2}{\epsilon_d} - 24 \log\left(\frac{r}{R_\theta}\right) \hat{n} \cdot \vec{v}_2 \hat{n} \cdot \vec{a}_1 \cdot \vec{S}_1 + 8 \hat{n} \cdot \vec{v}_2 \right. \\ & \left. \hat{n} \times \vec{a}_1 \cdot \vec{S}_1 + 8 \log\left(\frac{r}{R_\theta}\right) \vec{a}_1 \times \vec{S}_1 \cdot \vec{v}_2 + 24 \log\left(\frac{r}{R_\theta}\right) \hat{n} \cdot \vec{v}_2 \hat{n} \times \vec{S}_1 \cdot \vec{v}_1 - 8 \hat{n} \cdot \vec{v}_2 \hat{n} \times \vec{S}_1 \cdot \vec{v}_1 - 8 \log\left(\frac{r}{R_\theta}\right) \vec{S}_1 \times \vec{v}_1 \cdot \vec{v}_2 \right) + \\ & \frac{1}{r^4} G^3 m_2^3 \left( \frac{1}{\epsilon_d} \left( -8 (\hat{n} \cdot \vec{v}_2)^2 \hat{n} \times \vec{S}_1 \cdot \vec{v}_1 + \frac{16}{5} \hat{n} \cdot \vec{v}_2 \vec{S}_1 \times \vec{v}_1 \cdot \vec{v}_2 + 40 \hat{n} \cdot \vec{v}_1 \hat{n} \cdot \vec{v}_2 \hat{n} \times \vec{S}_1 \cdot \vec{v}_1 - 8 \hat{n} \cdot \vec{v}_1 \vec{S}_1 \times \vec{v}_1 \cdot \vec{v}_2 - \right. \right. \\ & \left. \left. 8 \vec{v}_1 \cdot \vec{v}_2 \hat{n} \times \vec{S}_1 \cdot \vec{v}_1 + \frac{8}{5} \vec{v}_2 \cdot \vec{v}_2 \hat{n} \times \vec{S}_1 \cdot \vec{v}_1 \right) + 24 \log\left(\frac{r}{R_\theta}\right) (\hat{n} \cdot \vec{v}_2)^2 \hat{n} \times \vec{S}_1 \cdot \vec{v}_1 - \frac{48}{5} \log\left(\frac{r}{R_\theta}\right) \hat{n} \cdot \vec{v}_2 \vec{S}_1 \times \vec{v}_1 \cdot \vec{v}_2 - \right. \\ & 120 \log\left(\frac{r}{R_\theta}\right) \hat{n} \cdot \vec{v}_1 \hat{n} \cdot \vec{v}_2 \hat{n} \times \vec{S}_1 \cdot \vec{v}_1 + 24 \log\left(\frac{r}{R_\theta}\right) \hat{n} \cdot \vec{v}_1 \vec{S}_1 \times \vec{v}_1 \cdot \vec{v}_2 + 24 \log\left(\frac{r}{R_\theta}\right) \vec{v}_1 \cdot \vec{v}_2 \hat{n} \times \vec{S}_1 \cdot \vec{v}_1 - \\ & \left. \frac{24}{5} \log\left(\frac{r}{R_\theta}\right) \vec{v}_2 \cdot \vec{v}_2 \hat{n} \times \vec{S}_1 \cdot \vec{v}_1 - 16 (\hat{n} \cdot \vec{v}_2)^2 \hat{n} \times \vec{S}_1 \cdot \vec{v}_1 + \frac{112}{25} \hat{n} \cdot \vec{v}_2 \vec{S}_1 \times \vec{v}_1 \cdot \vec{v}_2 + \right. \\ & \left. 64 \hat{n} \cdot \vec{v}_1 \hat{n} \cdot \vec{v}_2 \hat{n} \times \vec{S}_1 \cdot \vec{v}_1 - 8 \hat{n} \cdot \vec{v}_1 \vec{S}_1 \times \vec{v}_1 \cdot \vec{v}_2 - 8 \vec{v}_1 \cdot \vec{v}_2 \hat{n} \times \vec{S}_1 \cdot \vec{v}_1 + \frac{16}{25} \vec{v}_2 \cdot \vec{v}_2 \hat{n} \times \vec{S}_1 \cdot \vec{v}_1 \right) \Bigg\} \end{aligned}$$

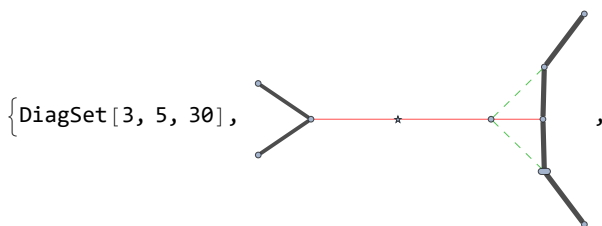

$$\begin{aligned}
& \frac{1}{r^3} G^3 m_1^2 m_2 \left( \frac{\frac{8}{5} \hat{n} \cdot \vec{v}_2 \hat{n} \times \vec{S}_1 \cdot \vec{a}_1 - \frac{8}{15} \vec{S}_1 \times \vec{a}_1 \cdot \vec{v}_2 + \frac{8}{5} \hat{n} \cdot \vec{v}_2 \hat{n} \times \vec{S}_1 \cdot \vec{v}_1 - \frac{8}{15} \vec{S}_1 \times \vec{v}_1 \cdot \vec{v}_2}{\epsilon_d} - \right. \\
& \frac{24}{5} \log\left(\frac{r}{R_\theta}\right) \hat{n} \cdot \vec{v}_2 \hat{n} \times \vec{S}_1 \cdot \vec{a}_1 + \frac{56}{25} \hat{n} \cdot \vec{v}_2 \hat{n} \times \vec{S}_1 \cdot \vec{a}_1 + \frac{8}{5} \log\left(\frac{r}{R_\theta}\right) \vec{S}_1 \times \vec{a}_1 \cdot \vec{v}_2 - \frac{16}{75} \vec{S}_1 \times \vec{a}_1 \cdot \vec{v}_2 - \\
& \left. \frac{24}{5} \log\left(\frac{r}{R_\theta}\right) \hat{n} \cdot \vec{v}_2 \hat{n} \times \vec{S}_1 \cdot \vec{v}_1 + \frac{56}{25} \hat{n} \cdot \vec{v}_2 \hat{n} \times \vec{S}_1 \cdot \vec{v}_1 + \frac{8}{5} \log\left(\frac{r}{R_\theta}\right) \vec{S}_1 \times \vec{v}_1 \cdot \vec{v}_2 - \frac{16}{75} \vec{S}_1 \times \vec{v}_1 \cdot \vec{v}_2 \right) + \frac{1}{r^4} \\
& G^3 m_1^2 m_2 \left( \frac{\frac{8}{5} \hat{n} \cdot \vec{v}_1 \vec{S}_1 \times \vec{v}_1 \cdot \vec{v}_2 - 8 \hat{n} \cdot \vec{v}_2 \hat{n} \cdot \vec{v}_1 \hat{n} \times \vec{S}_1 \cdot \vec{v}_1 + \frac{8}{5} \vec{v}_1 \cdot \vec{v}_2 \hat{n} \times \vec{S}_1 \cdot \vec{v}_1}{\epsilon_d} - \frac{24}{5} \log\left(\frac{r}{R_\theta}\right) \hat{n} \cdot \vec{v}_1 \vec{S}_1 \times \vec{v}_1 \cdot \vec{v}_2 + \right. \\
& 24 \log\left(\frac{r}{R_\theta}\right) \hat{n} \cdot \vec{v}_2 \hat{n} \cdot \vec{v}_1 \hat{n} \times \vec{S}_1 \cdot \vec{v}_1 - \frac{24}{5} \log\left(\frac{r}{R_\theta}\right) \vec{v}_1 \cdot \vec{v}_2 \hat{n} \times \vec{S}_1 \cdot \vec{v}_1 + \\
& \left. \frac{56}{25} \hat{n} \cdot \vec{v}_1 \vec{S}_1 \times \vec{v}_1 \cdot \vec{v}_2 - 16 \hat{n} \cdot \vec{v}_2 \hat{n} \cdot \vec{v}_1 \hat{n} \times \vec{S}_1 \cdot \vec{v}_1 + \frac{56}{25} \vec{v}_1 \cdot \vec{v}_2 \hat{n} \times \vec{S}_1 \cdot \vec{v}_1 \right) \}
\end{aligned}$$

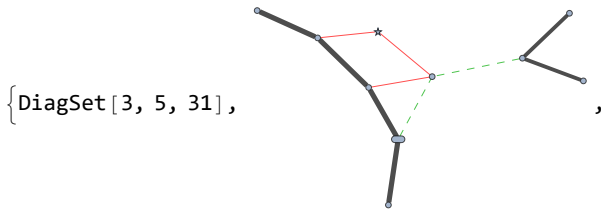

$$\begin{aligned}
& \frac{1}{r^3} m_1^2 m_2 \left( -\frac{32}{5} \log\left(\frac{r}{R_\theta}\right) \vec{S}_1 \times \vec{v}_1 \cdot \vec{v}_2 + \frac{64}{75} \vec{S}_1 \times \vec{v}_1 \cdot \vec{v}_2 + \frac{64}{75} \vec{S}_1 \times \vec{v}_1 \cdot \vec{a}_2 - \frac{88}{25} \hat{n} \times \vec{S}_1 \cdot \vec{v}_1 \hat{n} \cdot \vec{a}_2 - \frac{104}{25} \hat{n} \times \vec{S}_1 \cdot \vec{v}_2 \hat{n} \cdot \vec{v}_1 - \right. \\
& \frac{104}{25} \hat{n} \times \vec{S}_1 \cdot \vec{a}_2 \hat{n} \cdot \vec{v}_1 - \frac{88}{25} \hat{n} \times \vec{S}_1 \cdot \vec{v}_1 \hat{n} \cdot \vec{v}_2 - \frac{32}{5} \vec{S}_1 \times \vec{v}_1 \cdot \vec{a}_2 \log\left(\frac{r}{R_\theta}\right) + \frac{72}{5} \hat{n} \times \vec{S}_1 \cdot \vec{v}_1 \hat{n} \cdot \vec{a}_2 \log\left(\frac{r}{R_\theta}\right) - \\
& \frac{24}{5} \hat{n} \times \vec{S}_1 \cdot \vec{v}_2 \hat{n} \cdot \vec{v}_1 \log\left(\frac{r}{R_\theta}\right) - \frac{24}{5} \hat{n} \times \vec{S}_1 \cdot \vec{a}_2 \hat{n} \cdot \vec{v}_1 \log\left(\frac{r}{R_\theta}\right) + \frac{72}{5} \hat{n} \times \vec{S}_1 \cdot \vec{v}_1 \hat{n} \cdot \vec{v}_2 \log\left(\frac{r}{R_\theta}\right) + \frac{1}{\epsilon_d} \left( \frac{32}{15} \vec{S}_1 \times \vec{v}_1 \cdot \vec{v}_2 + \right. \\
& \left. \frac{32}{15} \vec{S}_1 \times \vec{v}_1 \cdot \vec{a}_2 - \frac{24}{5} \hat{n} \times \vec{S}_1 \cdot \vec{v}_1 \hat{n} \cdot \vec{a}_2 + \frac{8}{5} \hat{n} \times \vec{S}_1 \cdot \vec{v}_2 \hat{n} \cdot \vec{v}_1 + \frac{8}{5} \hat{n} \times \vec{S}_1 \cdot \vec{a}_2 \hat{n} \cdot \vec{v}_1 - \frac{24}{5} \hat{n} \times \vec{S}_1 \cdot \vec{v}_1 \hat{n} \cdot \vec{v}_2 \right) \Big) G^3 + \frac{1}{r^4} \\
& m_1^2 m_2 \left( \frac{736}{49} \hat{n} \times \vec{S}_1 \cdot \vec{v}_2 (\hat{n} \cdot \vec{v}_1)^2 + \frac{120}{7} \hat{n} \times \vec{S}_1 \cdot \vec{v}_2 \log\left(\frac{r}{R_\theta}\right) (\hat{n} \cdot \vec{v}_1)^2 + \frac{8}{49} \vec{S}_1 \times \vec{v}_1 \cdot \vec{v}_2 \hat{n} \cdot \vec{v}_1 + \frac{928}{49} \hat{n} \times \vec{S}_1 \cdot \vec{v}_1 \hat{n} \cdot \vec{v}_2 \hat{n} \cdot \vec{v}_1 - \right. \\
& 16 \hat{n} \times \vec{S}_1 \cdot \vec{v}_2 \hat{n} \cdot \vec{v}_2 \hat{n} \cdot \vec{v}_1 + \frac{120}{7} \vec{S}_1 \times \vec{v}_1 \cdot \vec{v}_2 \log\left(\frac{r}{R_\theta}\right) \hat{n} \cdot \vec{v}_1 - \frac{360}{7} \hat{n} \times \vec{S}_1 \cdot \vec{v}_1 \hat{n} \cdot \vec{v}_2 \log\left(\frac{r}{R_\theta}\right) \hat{n} \cdot \vec{v}_1 - \\
& 24 \hat{n} \times \vec{S}_1 \cdot \vec{v}_2 \hat{n} \cdot \vec{v}_2 \log\left(\frac{r}{R_\theta}\right) \hat{n} \cdot \vec{v}_1 - 32 \hat{n} \times \vec{S}_1 \cdot \vec{v}_1 (\hat{n} \cdot \vec{v}_2)^2 + \frac{312}{25} \vec{S}_1 \times \vec{v}_1 \cdot \vec{v}_2 \hat{n} \cdot \vec{v}_2 - \frac{8}{245} \hat{n} \times \vec{S}_1 \cdot \vec{v}_2 \vec{v}_1 \cdot \vec{v}_1 - \\
& \frac{152}{49} \hat{n} \times \vec{S}_1 \cdot \vec{v}_1 \vec{v}_1 \cdot \vec{v}_2 + \frac{104}{25} \hat{n} \times \vec{S}_1 \cdot \vec{v}_2 \vec{v}_1 \cdot \vec{v}_2 + \frac{88}{25} \hat{n} \times \vec{S}_1 \cdot \vec{v}_1 \vec{v}_2 \cdot \vec{v}_2 + 72 \hat{n} \times \vec{S}_1 \cdot \vec{v}_1 (\hat{n} \cdot \vec{v}_2)^2 \log\left(\frac{r}{R_\theta}\right) - \\
& \frac{168}{5} \vec{S}_1 \times \vec{v}_1 \cdot \vec{v}_2 \hat{n} \cdot \vec{v}_2 \log\left(\frac{r}{R_\theta}\right) - \frac{24}{7} \hat{n} \times \vec{S}_1 \cdot \vec{v}_2 \vec{v}_1 \cdot \vec{v}_1 \log\left(\frac{r}{R_\theta}\right) + \frac{72}{7} \hat{n} \times \vec{S}_1 \cdot \vec{v}_1 \vec{v}_1 \cdot \vec{v}_2 \log\left(\frac{r}{R_\theta}\right) + \\
& \frac{24}{5} \hat{n} \times \vec{S}_1 \cdot \vec{v}_2 \vec{v}_1 \cdot \vec{v}_2 \log\left(\frac{r}{R_\theta}\right) - \frac{72}{5} \hat{n} \times \vec{S}_1 \cdot \vec{v}_1 \vec{v}_2 \cdot \vec{v}_2 \log\left(\frac{r}{R_\theta}\right) + \frac{1}{\epsilon_d} \left( -\frac{40}{7} \hat{n} \times \vec{S}_1 \cdot \vec{v}_2 (\hat{n} \cdot \vec{v}_1)^2 - \right. \\
& \frac{40}{7} \vec{S}_1 \times \vec{v}_1 \cdot \vec{v}_2 \hat{n} \cdot \vec{v}_1 + \frac{120}{7} \hat{n} \times \vec{S}_1 \cdot \vec{v}_1 \hat{n} \cdot \vec{v}_2 \hat{n} \cdot \vec{v}_1 + 8 \hat{n} \times \vec{S}_1 \cdot \vec{v}_2 \hat{n} \cdot \vec{v}_2 \hat{n} \cdot \vec{v}_1 - 24 \hat{n} \times \vec{S}_1 \cdot \vec{v}_1 (\hat{n} \cdot \vec{v}_2)^2 + \\
& \left. \frac{56}{5} \vec{S}_1 \times \vec{v}_1 \cdot \vec{v}_2 \hat{n} \cdot \vec{v}_2 + \frac{8}{7} \hat{n} \times \vec{S}_1 \cdot \vec{v}_2 \vec{v}_1 \cdot \vec{v}_1 - \frac{24}{7} \hat{n} \times \vec{S}_1 \cdot \vec{v}_1 \vec{v}_1 \cdot \vec{v}_2 - \frac{8}{5} \hat{n} \times \vec{S}_1 \cdot \vec{v}_2 \vec{v}_1 \cdot \vec{v}_2 + \frac{24}{5} \hat{n} \times \vec{S}_1 \cdot \vec{v}_1 \vec{v}_2 \cdot \vec{v}_2 \right) \Big) G^3 \}
\end{aligned}$$



$\{\text{DiagSet}[3, 5, 32],$  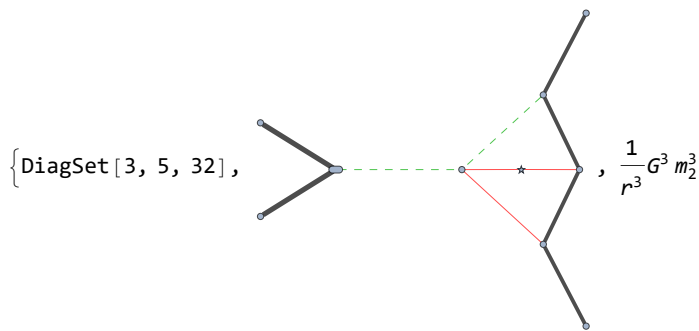  $, \frac{1}{r^3} G^3 m_2^3$

$$\left( \frac{-8 \hat{n} \cdot \vec{a}_2 \hat{n} \times \vec{S}_1 \cdot \vec{v}_2 - 8 \hat{n} \cdot \vec{v}_2 \hat{n} \times \vec{a}_2 \cdot \vec{S}_1 + \frac{16}{3} \vec{a}_2 \times \vec{S}_1 \cdot \vec{v}_2}{\epsilon_d} + 24 \log\left(\frac{r}{R_\theta}\right) \hat{n} \cdot \vec{a}_2 \hat{n} \times \vec{S}_1 \cdot \vec{v}_2 + 24 \log\left(\frac{r}{R_\theta}\right) \hat{n} \cdot \vec{v}_2 \hat{n} \times \vec{a}_2 \cdot \vec{S}_1 - \right.$$

$$8 \hat{n} \cdot \vec{a}_2 \hat{n} \times \vec{S}_1 \cdot \vec{v}_2 - 24 \hat{n} \cdot \vec{v}_2 \hat{n} \times \vec{a}_2 \cdot \vec{S}_1 - 16 \log\left(\frac{r}{R_\theta}\right) \vec{a}_2 \times \vec{S}_1 \cdot \vec{v}_2 + \frac{16}{3} \vec{a}_2 \times \vec{S}_1 \cdot \vec{v}_2 + 16 \hat{n} \cdot \vec{v}_2 \hat{n} \times \vec{S}_1 \cdot \vec{v}_2 \left. \right) +$$

$$\frac{1}{r^4} G^3 m_2^3 \left( 64 (\hat{n} \cdot \vec{v}_2)^2 \hat{n} \times \vec{S}_1 \cdot \vec{v}_2 - 16 \hat{n} \cdot \vec{v}_2 \vec{S}_1 \times \vec{v}_1 \cdot \vec{v}_2 - 80 \hat{n} \cdot \vec{v}_1 \hat{n} \cdot \vec{v}_2 \hat{n} \times \vec{S}_1 \cdot \vec{v}_2 + 16 \vec{v}_1 \cdot \vec{v}_2 \hat{n} \times \vec{S}_1 \cdot \vec{v}_2 \right) \}$$

$\{\text{DiagSet}[3, 5, 33],$  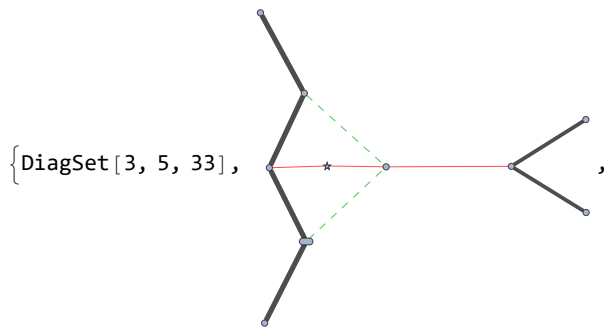  $,$

$$\frac{1}{r^3} G^3 m_1^2 m_2 \left( \frac{\frac{8}{5} \hat{n} \cdot \vec{v}_1 \hat{n} \times \vec{S}_1 \cdot \vec{a}_1 + \frac{8}{15} \vec{S}_1 \times \vec{v}_1 \cdot \vec{a}_1 + \frac{8}{5} \hat{n} \cdot \vec{v}_1 \hat{n} \times \vec{S}_1 \cdot \vec{v}_1}{\epsilon_d} - \frac{24}{5} \log\left(\frac{r}{R_\theta}\right) \hat{n} \cdot \vec{v}_1 \hat{n} \times \vec{S}_1 \cdot \vec{a}_1 + \frac{96}{25} \hat{n} \cdot \vec{v}_1 \hat{n} \times \vec{S}_1 \cdot \vec{a}_1 - \right.$$

$$\left. \frac{8}{5} \log\left(\frac{r}{R_\theta}\right) \vec{S}_1 \times \vec{v}_1 \cdot \vec{a}_1 + \frac{16}{75} \vec{S}_1 \times \vec{v}_1 \cdot \vec{a}_1 - \frac{24}{5} \log\left(\frac{r}{R_\theta}\right) \hat{n} \cdot \vec{v}_1 \hat{n} \times \vec{S}_1 \cdot \vec{v}_1 + \frac{96}{25} \hat{n} \cdot \vec{v}_1 \hat{n} \times \vec{S}_1 \cdot \vec{v}_1 \right) + \frac{1}{r^4}$$

$$G^3 m_1^2 m_2 \left( \frac{1}{\epsilon_d} \left( -\frac{48}{7} (\hat{n} \cdot \vec{v}_1)^2 \hat{n} \times \vec{S}_1 \cdot \vec{v}_1 - \frac{8}{5} \hat{n} \cdot \vec{v}_1 \vec{S}_1 \times \vec{v}_1 \cdot \vec{v}_2 + 8 \hat{n} \cdot \vec{v}_2 \hat{n} \cdot \vec{v}_1 \hat{n} \times \vec{S}_1 \cdot \vec{v}_1 + \frac{48}{35} \vec{v}_1 \cdot \vec{v}_1 \hat{n} \times \vec{S}_1 \cdot \vec{v}_1 - \right. \right.$$

$$\left. \frac{8}{5} \vec{v}_1 \cdot \vec{v}_2 \hat{n} \times \vec{S}_1 \cdot \vec{v}_1 \right) + \frac{144}{7} \log\left(\frac{r}{R_\theta}\right) (\hat{n} \cdot \vec{v}_1)^2 \hat{n} \times \vec{S}_1 \cdot \vec{v}_1 + \frac{24}{5} \log\left(\frac{r}{R_\theta}\right) \hat{n} \cdot \vec{v}_1 \vec{S}_1 \times \vec{v}_1 \cdot \vec{v}_2 - 24 \log\left(\frac{r}{R_\theta}\right) \hat{n} \cdot \vec{v}_2$$

$$\hat{n} \cdot \vec{v}_1 \hat{n} \times \vec{S}_1 \cdot \vec{v}_1 - \frac{144}{35} \log\left(\frac{r}{R_\theta}\right) \vec{v}_1 \cdot \vec{v}_1 \hat{n} \times \vec{S}_1 \cdot \vec{v}_1 + \frac{24}{5} \log\left(\frac{r}{R_\theta}\right) \vec{v}_1 \cdot \vec{v}_2 \hat{n} \times \vec{S}_1 \cdot \vec{v}_1 - \frac{976}{49} (\hat{n} \cdot \vec{v}_1)^2 \hat{n} \times \vec{S}_1 \cdot \vec{v}_1 -$$

$$\left. \frac{96}{25} \hat{n} \cdot \vec{v}_1 \vec{S}_1 \times \vec{v}_1 \cdot \vec{v}_2 + 24 \hat{n} \cdot \vec{v}_2 \hat{n} \cdot \vec{v}_1 \hat{n} \times \vec{S}_1 \cdot \vec{v}_1 + \frac{2192 \vec{v}_1 \cdot \vec{v}_1 \hat{n} \times \vec{S}_1 \cdot \vec{v}_1}{1225} - \frac{96}{25} \vec{v}_1 \cdot \vec{v}_2 \hat{n} \times \vec{S}_1 \cdot \vec{v}_1 \right) \}$$

$\{\text{DiagSet}[3, 5, 34],$  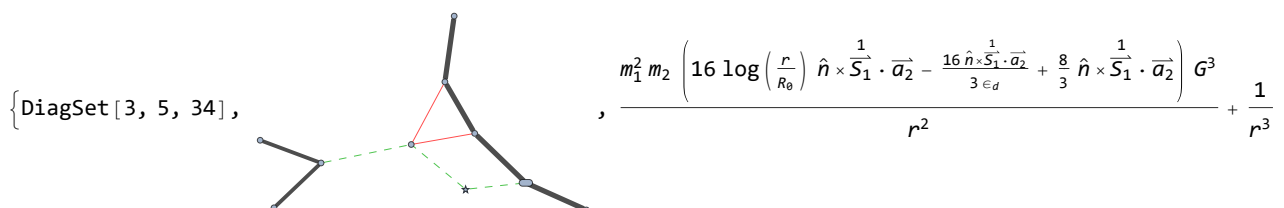  $, \frac{m_1^2 m_2 \left( 16 \log\left(\frac{r}{R_\theta}\right) \hat{n} \times \vec{S}_1 \cdot \vec{a}_2 - \frac{16 \hat{n} \times \vec{S}_1 \cdot \vec{a}_2}{3 \epsilon_d} + \frac{8}{3} \hat{n} \times \vec{S}_1 \cdot \vec{a}_2 \right) G^3}{r^2} + \frac{1}{r^3}$

$$\begin{aligned}
& m_1^2 m_2 \left( -\frac{64}{5} \log\left(\frac{r}{R_0}\right) \frac{1}{S_1} \times \vec{v}_1 \cdot \vec{v}_2 - \frac{32}{75} \frac{1}{S_1} \times \vec{v}_1 \cdot \vec{v}_2 - \frac{56}{25} \vec{S}_1 \times \vec{v}_1 \cdot \vec{a}_2 + \frac{56}{25} \hat{n} \times \vec{S}_1 \cdot \vec{v}_1 \hat{n} \cdot \vec{a}_2 + \frac{152}{25} \hat{n} \times \vec{S}_1 \cdot \vec{v}_2 \hat{n} \cdot \vec{v}_1 + \right. \\
& \frac{48}{25} \hat{n} \times \vec{S}_1 \cdot \vec{a}_2 \hat{n} \cdot \vec{v}_1 - \frac{56}{25} \hat{n} \times \vec{S}_1 \cdot \vec{v}_1 \hat{n} \cdot \vec{v}_2 - 8 \hat{n} \times \vec{S}_1 \cdot \vec{v}_2 \hat{n} \cdot \vec{v}_2 - \frac{16}{5} \vec{S}_1 \times \vec{v}_1 \cdot \vec{a}_2 \log\left(\frac{r}{R_0}\right) - \\
& \frac{24}{5} \hat{n} \times \vec{S}_1 \cdot \vec{v}_1 \hat{n} \cdot \vec{a}_2 \log\left(\frac{r}{R_0}\right) - \frac{168}{5} \hat{n} \times \vec{S}_1 \cdot \vec{v}_2 \hat{n} \cdot \vec{v}_1 \log\left(\frac{r}{R_0}\right) - \frac{72}{5} \hat{n} \times \vec{S}_1 \cdot \vec{a}_2 \hat{n} \cdot \vec{v}_1 \log\left(\frac{r}{R_0}\right) + \\
& \frac{24}{5} \hat{n} \times \vec{S}_1 \cdot \vec{v}_1 \hat{n} \cdot \vec{v}_2 \log\left(\frac{r}{R_0}\right) + 48 \hat{n} \times \vec{S}_1 \cdot \vec{v}_2 \hat{n} \cdot \vec{v}_2 \log\left(\frac{r}{R_0}\right) + \frac{1}{\epsilon_d} \left( \frac{64}{15} \vec{S}_1 \times \vec{v}_1 \cdot \vec{v}_2 + \frac{16}{15} \vec{S}_1 \times \vec{v}_1 \cdot \vec{a}_2 + \right. \\
& \left. \frac{8}{5} \hat{n} \times \vec{S}_1 \cdot \vec{v}_1 \hat{n} \cdot \vec{a}_2 + \frac{56}{5} \hat{n} \times \vec{S}_1 \cdot \vec{v}_2 \hat{n} \cdot \vec{v}_1 + \frac{24}{5} \hat{n} \times \vec{S}_1 \cdot \vec{a}_2 \hat{n} \cdot \vec{v}_1 - \frac{8}{5} \hat{n} \times \vec{S}_1 \cdot \vec{v}_1 \hat{n} \cdot \vec{v}_2 - 16 \hat{n} \times \vec{S}_1 \cdot \vec{v}_2 \hat{n} \cdot \vec{v}_2 \right) \Bigg) G^3 + \\
& \frac{1}{r^4} m_1^2 m_2 \left( -\frac{736}{49} \hat{n} \times \vec{S}_1 \cdot \vec{v}_2 (\hat{n} \cdot \vec{v}_1)^2 + \frac{216}{7} \hat{n} \times \vec{S}_1 \cdot \vec{v}_2 \log\left(\frac{r}{R_0}\right) (\hat{n} \cdot \vec{v}_1)^2 - \frac{984 \vec{S}_1 \times \vec{v}_1 \cdot \vec{v}_2 \hat{n} \cdot \vec{v}_1}{1225} - \right. \\
& \frac{144}{49} \hat{n} \times \vec{S}_1 \cdot \vec{v}_1 \hat{n} \cdot \vec{v}_2 \hat{n} \cdot \vec{v}_1 + 24 \hat{n} \times \vec{S}_1 \cdot \vec{v}_2 \hat{n} \cdot \vec{v}_2 \hat{n} \cdot \vec{v}_1 + \frac{408}{35} \vec{S}_1 \times \vec{v}_1 \cdot \vec{v}_2 \log\left(\frac{r}{R_0}\right) \hat{n} \cdot \vec{v}_1 + \\
& \frac{24}{7} \hat{n} \times \vec{S}_1 \cdot \vec{v}_1 \hat{n} \cdot \vec{v}_2 \log\left(\frac{r}{R_0}\right) \hat{n} \cdot \vec{v}_1 - 72 \hat{n} \times \vec{S}_1 \cdot \vec{v}_2 \hat{n} \cdot \vec{v}_2 \log\left(\frac{r}{R_0}\right) \hat{n} \cdot \vec{v}_1 + 16 \hat{n} \times \vec{S}_1 \cdot \vec{v}_1 (\hat{n} \cdot \vec{v}_2)^2 - \\
& \frac{144}{25} \vec{S}_1 \times \vec{v}_1 \cdot \vec{v}_2 \hat{n} \cdot \vec{v}_2 + \frac{1608 \hat{n} \times \vec{S}_1 \cdot \vec{v}_2 \vec{v}_1 \cdot \vec{v}_1}{1225} - \frac{1688 \hat{n} \times \vec{S}_1 \cdot \vec{v}_1 \vec{v}_1 \cdot \vec{v}_2}{1225} - \frac{48}{25} \hat{n} \times \vec{S}_1 \cdot \vec{v}_2 \vec{v}_1 \cdot \vec{v}_2 - \\
& \frac{56}{25} \hat{n} \times \vec{S}_1 \cdot \vec{v}_1 \vec{v}_2 \cdot \vec{v}_2 - 24 \hat{n} \times \vec{S}_1 \cdot \vec{v}_1 (\hat{n} \cdot \vec{v}_2)^2 \log\left(\frac{r}{R_0}\right) - \frac{24}{5} \vec{S}_1 \times \vec{v}_1 \cdot \vec{v}_2 \hat{n} \cdot \vec{v}_2 \log\left(\frac{r}{R_0}\right) - \\
& \frac{216}{35} \hat{n} \times \vec{S}_1 \cdot \vec{v}_2 \vec{v}_1 \cdot \vec{v}_1 \log\left(\frac{r}{R_0}\right) - \frac{24}{35} \hat{n} \times \vec{S}_1 \cdot \vec{v}_1 \vec{v}_1 \cdot \vec{v}_2 \log\left(\frac{r}{R_0}\right) + \frac{72}{5} \hat{n} \times \vec{S}_1 \cdot \vec{v}_2 \vec{v}_1 \cdot \vec{v}_2 \log\left(\frac{r}{R_0}\right) + \\
& \frac{24}{5} \hat{n} \times \vec{S}_1 \cdot \vec{v}_1 \vec{v}_2 \cdot \vec{v}_2 \log\left(\frac{r}{R_0}\right) + \frac{1}{\epsilon_d} \left( -\frac{72}{7} \hat{n} \times \vec{S}_1 \cdot \vec{v}_2 (\hat{n} \cdot \vec{v}_1)^2 - \frac{136}{35} \vec{S}_1 \times \vec{v}_1 \cdot \vec{v}_2 \hat{n} \cdot \vec{v}_1 - \right. \\
& \left. \frac{8}{7} \hat{n} \times \vec{S}_1 \cdot \vec{v}_1 \hat{n} \cdot \vec{v}_2 \hat{n} \cdot \vec{v}_1 + 24 \hat{n} \times \vec{S}_1 \cdot \vec{v}_2 \hat{n} \cdot \vec{v}_2 \hat{n} \cdot \vec{v}_1 + 8 \hat{n} \times \vec{S}_1 \cdot \vec{v}_1 (\hat{n} \cdot \vec{v}_2)^2 + \frac{8}{5} \vec{S}_1 \times \vec{v}_1 \cdot \vec{v}_2 \hat{n} \cdot \vec{v}_2 + \right. \\
& \left. \frac{72}{35} \hat{n} \times \vec{S}_1 \cdot \vec{v}_2 \vec{v}_1 \cdot \vec{v}_1 + \frac{8}{35} \hat{n} \times \vec{S}_1 \cdot \vec{v}_1 \vec{v}_1 \cdot \vec{v}_2 - \frac{24}{5} \hat{n} \times \vec{S}_1 \cdot \vec{v}_2 \vec{v}_1 \cdot \vec{v}_2 - \frac{8}{5} \hat{n} \times \vec{S}_1 \cdot \vec{v}_1 \vec{v}_2 \cdot \vec{v}_2 \right) \Bigg) G^3 \Bigg\}
\end{aligned}$$

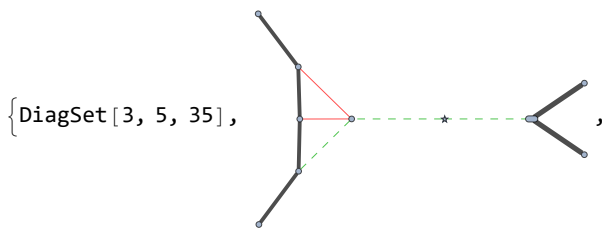

$$\begin{aligned}
& \frac{1}{r^3} G^3 m_2^3 \left( \frac{-8 \hat{n} \cdot \vec{v}_1 \hat{n} \times \vec{a}_2 \cdot \vec{S}_1 + \frac{8}{3} \vec{a}_2 \times \vec{S}_1 \cdot \vec{v}_1 - 8 \hat{n} \cdot \vec{v}_2 \hat{n} \times \vec{S}_1 \cdot \vec{v}_2}{\epsilon_d} + 24 \log\left(\frac{r}{R_0}\right) \hat{n} \cdot \vec{v}_1 \hat{n} \times \vec{a}_2 \cdot \vec{S}_1 - \right. \\
& \left. 8 \hat{n} \cdot \vec{v}_1 \hat{n} \times \vec{a}_2 \cdot \vec{S}_1 - 8 \log\left(\frac{r}{R_0}\right) \vec{a}_2 \times \vec{S}_1 \cdot \vec{v}_1 + 24 \log\left(\frac{r}{R_0}\right) \hat{n} \cdot \vec{v}_2 \hat{n} \times \vec{S}_1 \cdot \vec{v}_2 - 8 \hat{n} \cdot \vec{v}_2 \hat{n} \times \vec{S}_1 \cdot \vec{v}_2 \right) + \\
& \frac{G^3 m_2^3 \left( \frac{8 \hat{n} \times \vec{a}_2 \cdot \vec{S}_1}{3 \epsilon_d} - 8 \log\left(\frac{r}{R_0}\right) \hat{n} \times \vec{a}_2 \cdot \vec{S}_1 \right)}{r^2} + \frac{1}{r^4} G^3 m_2^3 \left( \frac{8 \hat{n} \cdot \vec{v}_2 \vec{S}_1 \times \vec{v}_1 \cdot \vec{v}_2 + 40 \hat{n} \cdot \vec{v}_1 \hat{n} \cdot \vec{v}_2 \hat{n} \times \vec{S}_1 \cdot \vec{v}_2 - 8 \vec{v}_1 \cdot \vec{v}_2 \hat{n} \times \vec{S}_1 \cdot \vec{v}_2}{\epsilon_d} - \right. \\
& \left. 24 \log\left(\frac{r}{R_0}\right) \hat{n} \cdot \vec{v}_2 \vec{S}_1 \times \vec{v}_1 \cdot \vec{v}_2 - 120 \log\left(\frac{r}{R_0}\right) \hat{n} \cdot \vec{v}_1 \hat{n} \cdot \vec{v}_2 \hat{n} \times \vec{S}_1 \cdot \vec{v}_2 + \right.
\end{aligned}$$

$$24 \log \left( \frac{r}{R_0} \right) \vec{v}_1 \cdot \vec{v}_2 \hat{n} \times \vec{S}_1 \cdot \vec{v}_2 + 8 \hat{n} \cdot \vec{v}_2 \vec{S}_1 \times \vec{v}_1 \cdot \vec{v}_2 + 64 \hat{n} \cdot \vec{v}_1 \hat{n} \cdot \vec{v}_2 \hat{n} \times \vec{S}_1 \cdot \vec{v}_2 - 8 \vec{v}_1 \cdot \vec{v}_2 \hat{n} \times \vec{S}_1 \cdot \vec{v}_2 \Big\}$$

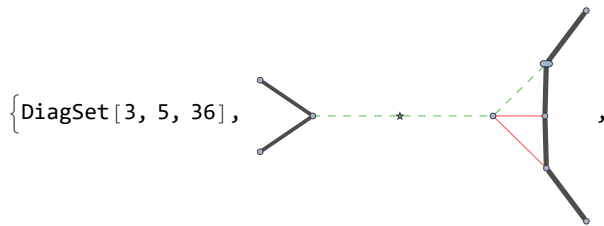

$$\frac{1}{r^3} G^3 m_1^2 m_2 \left( \frac{\frac{8}{5} \hat{n} \cdot \vec{v}_1 \hat{n} \times \vec{S}_1 \cdot \vec{a}_2 + \frac{8}{15} \vec{S}_1 \times \vec{v}_1 \cdot \vec{a}_2 - \frac{8}{5} \hat{n} \cdot \vec{v}_2 \hat{n} \times \vec{S}_1 \cdot \vec{v}_2}{\epsilon_d} - \frac{24}{5} \log \left( \frac{r}{R_0} \right) \hat{n} \cdot \vec{v}_1 \hat{n} \times \vec{S}_1 \cdot \vec{a}_2 + \frac{56}{25} \hat{n} \cdot \vec{v}_1 \hat{n} \times \vec{S}_1 \cdot \vec{a}_2 - \right.$$

$$\left. \frac{8}{5} \log \left( \frac{r}{R_0} \right) \vec{S}_1 \times \vec{v}_1 \cdot \vec{a}_2 + \frac{16}{75} \vec{S}_1 \times \vec{v}_1 \cdot \vec{a}_2 + \frac{24}{5} \log \left( \frac{r}{R_0} \right) \hat{n} \cdot \vec{v}_2 \hat{n} \times \vec{S}_1 \cdot \vec{v}_2 - \frac{56}{25} \hat{n} \cdot \vec{v}_2 \hat{n} \times \vec{S}_1 \cdot \vec{v}_2 \right) +$$

$$\frac{G^3 m_1^2 m_2 \left( -\frac{8 \hat{n} \times \vec{S}_1 \cdot \vec{a}_2}{15 \epsilon_d} + \frac{8}{5} \log \left( \frac{r}{R_0} \right) \hat{n} \times \vec{S}_1 \cdot \vec{a}_2 - \frac{16}{75} \hat{n} \times \vec{S}_1 \cdot \vec{a}_2 \right)}{r^2} + \frac{1}{r^4}$$

$$G^3 m_1^2 m_2 \left( \frac{\frac{8}{5} \hat{n} \cdot \vec{v}_2 \vec{S}_1 \times \vec{v}_1 \cdot \vec{v}_2 + 8 \hat{n} \cdot \vec{v}_1 \hat{n} \cdot \vec{v}_2 \hat{n} \times \vec{S}_1 \cdot \vec{v}_2 - \frac{8}{5} \vec{v}_1 \cdot \vec{v}_2 \hat{n} \times \vec{S}_1 \cdot \vec{v}_2}{\epsilon_d} - \right.$$

$$\left. \frac{24}{5} \log \left( \frac{r}{R_0} \right) \hat{n} \cdot \vec{v}_2 \vec{S}_1 \times \vec{v}_1 \cdot \vec{v}_2 - 24 \log \left( \frac{r}{R_0} \right) \hat{n} \cdot \vec{v}_1 \hat{n} \cdot \vec{v}_2 \hat{n} \times \vec{S}_1 \cdot \vec{v}_2 + \frac{24}{5} \log \left( \frac{r}{R_0} \right) \vec{v}_1 \cdot \vec{v}_2 \hat{n} \times \vec{S}_1 \cdot \vec{v}_2 + \right.$$

$$\left. \frac{56}{25} \hat{n} \cdot \vec{v}_2 \vec{S}_1 \times \vec{v}_1 \cdot \vec{v}_2 + 16 \hat{n} \cdot \vec{v}_1 \hat{n} \cdot \vec{v}_2 \hat{n} \times \vec{S}_1 \cdot \vec{v}_2 - \frac{56}{25} \vec{v}_1 \cdot \vec{v}_2 \hat{n} \times \vec{S}_1 \cdot \vec{v}_2 \right\}$$

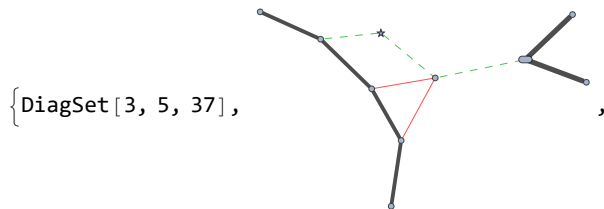

$$\frac{1}{r^3} G^3 m_2^3 \left( \frac{-8 \hat{n} \cdot \vec{a}_2 \hat{n} \times \vec{S}_1 \cdot \vec{v}_2 - 8 \hat{n} \cdot \vec{v}_2 \hat{n} \times \vec{a}_2 \cdot \vec{S}_1 + \frac{16}{3} \vec{a}_2 \times \vec{S}_1 \cdot \vec{v}_2}{\epsilon_d} + 24 \log \left( \frac{r}{R_0} \right) \hat{n} \cdot \vec{a}_2 \hat{n} \times \vec{S}_1 \cdot \vec{v}_2 + \right.$$

$$24 \log \left( \frac{r}{R_0} \right) \hat{n} \cdot \vec{v}_2 \hat{n} \times \vec{a}_2 \cdot \vec{S}_1 - 8 \hat{n} \cdot \vec{a}_2 \hat{n} \times \vec{S}_1 \cdot \vec{v}_2 + 24 \hat{n} \cdot \vec{v}_1 \hat{n} \times \vec{a}_2 \cdot \vec{S}_1 - 24 \hat{n} \cdot \vec{v}_2 \hat{n} \times \vec{a}_2 \cdot \vec{S}_1 -$$

$$16 \log \left( \frac{r}{R_0} \right) \vec{a}_2 \times \vec{S}_1 \cdot \vec{v}_2 - 8 \vec{a}_2 \times \vec{S}_1 \cdot \vec{v}_1 + \frac{16}{3} \vec{a}_2 \times \vec{S}_1 \cdot \vec{v}_2 + 8 \hat{n} \cdot \vec{v}_2 \hat{n} \times \vec{S}_1 \cdot \vec{v}_2 \Big) - \frac{8 G^3 m_2^3 \hat{n} \times \vec{a}_2 \cdot \vec{S}_1}{r^2} +$$

$$\frac{1}{r^4} G^3 m_2^3 \left( 16 (\hat{n} \cdot \vec{v}_2)^2 \hat{n} \times \vec{S}_1 \cdot \vec{v}_2 - 8 \hat{n} \cdot \vec{v}_2 \vec{S}_1 \times \vec{v}_1 \cdot \vec{v}_2 - 40 \hat{n} \cdot \vec{v}_1 \hat{n} \cdot \vec{v}_2 \hat{n} \times \vec{S}_1 \cdot \vec{v}_2 + 8 \vec{v}_1 \cdot \vec{v}_2 \hat{n} \times \vec{S}_1 \cdot \vec{v}_2 \right) \Big\}$$

{DiagSet[3, 5, 38],

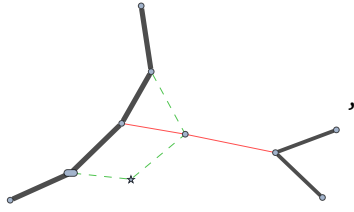

$$\frac{m_1^2 m_2 \left( -8 \log\left(\frac{r}{R_\theta}\right) \hat{n} \times \vec{S}_1 \cdot \vec{a}_1 + \frac{8 \hat{n} \times \vec{S}_1 \cdot \vec{a}_1}{3 \in_d} - \frac{8}{3} \hat{n} \times \vec{S}_1 \cdot \vec{a}_1 \right) G^3}{r^2} + \frac{1}{r^3} m_1^2 m_2 \left( 8 \log\left(\frac{r}{R_\theta}\right) \vec{S}_1 \times \vec{v}_1 \cdot \vec{v}_2 + \frac{8}{3} \vec{S}_1 \times \vec{v}_1 \cdot \vec{v}_2 + \right. \\ \left. \frac{72}{25} \vec{S}_1 \times \vec{v}_1 \cdot \vec{a}_1 - \frac{56}{25} \hat{n} \times \vec{S}_1 \cdot \vec{v}_1 \hat{n} \cdot \vec{a}_1 + \frac{16}{25} \hat{n} \times \vec{S}_1 \cdot \vec{v}_1 \hat{n} \cdot \vec{v}_1 + \frac{8}{5} \hat{n} \times \vec{S}_1 \cdot \vec{a}_1 \hat{n} \cdot \vec{v}_1 - \frac{8}{5} \vec{S}_1 \times \vec{v}_1 \cdot \vec{a}_1 \log\left(\frac{r}{R_\theta}\right) + \right. \\ \left. \frac{24}{5} \hat{n} \times \vec{S}_1 \cdot \vec{v}_1 \hat{n} \cdot \vec{a}_1 \log\left(\frac{r}{R_\theta}\right) + \frac{96}{5} \hat{n} \times \vec{S}_1 \cdot \vec{v}_1 \hat{n} \cdot \vec{v}_1 \log\left(\frac{r}{R_\theta}\right) - 24 \hat{n} \times \vec{S}_1 \cdot \vec{v}_1 \hat{n} \cdot \vec{v}_2 \log\left(\frac{r}{R_\theta}\right) + \frac{1}{\epsilon_d} \right. \\ \left. \left( -\frac{8}{3} \vec{S}_1 \times \vec{v}_1 \cdot \vec{v}_2 + \frac{8}{15} \vec{S}_1 \times \vec{v}_1 \cdot \vec{a}_1 - \frac{8}{5} \hat{n} \times \vec{S}_1 \cdot \vec{v}_1 \hat{n} \cdot \vec{a}_1 - \frac{32}{5} \hat{n} \times \vec{S}_1 \cdot \vec{v}_1 \hat{n} \cdot \vec{v}_1 + 8 \hat{n} \times \vec{S}_1 \cdot \vec{v}_1 \hat{n} \cdot \vec{v}_2 \right) \right) G^3 + \frac{1}{r^4} \\ m_1^2 m_2 \left( \frac{240}{49} \hat{n} \times \vec{S}_1 \cdot \vec{v}_1 (\hat{n} \cdot \vec{v}_1)^2 - \frac{96}{7} \hat{n} \times \vec{S}_1 \cdot \vec{v}_1 \log\left(\frac{r}{R_\theta}\right) (\hat{n} \cdot \vec{v}_1)^2 + \frac{16}{25} \vec{S}_1 \times \vec{v}_1 \cdot \vec{v}_2 \hat{n} \cdot \vec{v}_1 - 8 \hat{n} \times \vec{S}_1 \cdot \vec{v}_1 \hat{n} \cdot \vec{v}_2 \hat{n} \cdot \vec{v}_1 - \right. \\ \left. \frac{24}{5} \vec{S}_1 \times \vec{v}_1 \cdot \vec{v}_2 \log\left(\frac{r}{R_\theta}\right) \hat{n} \cdot \vec{v}_1 + 24 \hat{n} \times \vec{S}_1 \cdot \vec{v}_1 \hat{n} \cdot \vec{v}_2 \log\left(\frac{r}{R_\theta}\right) \hat{n} \cdot \vec{v}_1 + \frac{592 \hat{n} \times \vec{S}_1 \cdot \vec{v}_1 \vec{v}_1 \cdot \vec{v}_1}{1225} + \frac{16}{25} \hat{n} \times \vec{S}_1 \cdot \vec{v}_1 \vec{v}_1 \cdot \vec{v}_2 + \right. \\ \left. \frac{96}{35} \hat{n} \times \vec{S}_1 \cdot \vec{v}_1 \vec{v}_1 \cdot \vec{v}_1 \log\left(\frac{r}{R_\theta}\right) - \frac{24}{5} \hat{n} \times \vec{S}_1 \cdot \vec{v}_1 \vec{v}_1 \cdot \vec{v}_2 \log\left(\frac{r}{R_\theta}\right) + \frac{1}{\epsilon_d} \left( \frac{32}{7} \hat{n} \times \vec{S}_1 \cdot \vec{v}_1 (\hat{n} \cdot \vec{v}_1)^2 + \right. \right. \\ \left. \left. \frac{8}{5} \vec{S}_1 \times \vec{v}_1 \cdot \vec{v}_2 \hat{n} \cdot \vec{v}_1 - 8 \hat{n} \times \vec{S}_1 \cdot \vec{v}_1 \hat{n} \cdot \vec{v}_2 \hat{n} \cdot \vec{v}_1 - \frac{32}{35} \hat{n} \times \vec{S}_1 \cdot \vec{v}_1 \vec{v}_1 \cdot \vec{v}_1 + \frac{8}{5} \hat{n} \times \vec{S}_1 \cdot \vec{v}_1 \vec{v}_1 \cdot \vec{v}_2 \right) \right) G^3 \Big\}$$

{DiagSet[3, 5, 39],

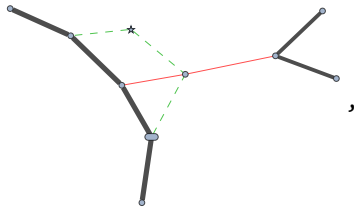

$$\frac{m_1^2 m_2 \left( 8 \log\left(\frac{r}{R_\theta}\right) \hat{n} \times \vec{S}_1 \cdot \vec{a}_1 - \frac{8 \hat{n} \times \vec{S}_1 \cdot \vec{a}_1}{3 \in_d} - \frac{8}{3} \hat{n} \times \vec{S}_1 \cdot \vec{a}_1 \right) G^3}{r^2} + \frac{1}{r^3} \\ m_1^2 m_2 \left( -8 \log\left(\frac{r}{R_\theta}\right) \vec{S}_1 \times \vec{a}_1 \cdot \vec{v}_2 + \frac{8}{3} \vec{S}_1 \times \vec{a}_1 \cdot \vec{v}_2 + \frac{56}{15} \vec{S}_1 \times \vec{v}_1 \cdot \vec{a}_1 - \frac{88}{25} \hat{n} \times \vec{S}_1 \cdot \vec{v}_1 \hat{n} \cdot \vec{a}_1 + \frac{96}{25} \hat{n} \times \vec{S}_1 \cdot \vec{v}_1 \hat{n} \cdot \vec{v}_1 + \right. \\ \left. \frac{392}{25} \hat{n} \times \vec{S}_1 \cdot \vec{a}_1 \hat{n} \cdot \vec{v}_1 - 16 \hat{n} \times \vec{S}_1 \cdot \vec{a}_1 \hat{n} \cdot \vec{v}_2 - 16 \vec{S}_1 \times \vec{v}_1 \cdot \vec{a}_1 \log\left(\frac{r}{R_\theta}\right) + \frac{72}{5} \hat{n} \times \vec{S}_1 \cdot \vec{v}_1 \hat{n} \cdot \vec{a}_1 \log\left(\frac{r}{R_\theta}\right) - \right. \\ \left. \frac{24}{5} \hat{n} \times \vec{S}_1 \cdot \vec{v}_1 \hat{n} \cdot \vec{v}_1 \log\left(\frac{r}{R_\theta}\right) - \frac{168}{5} \hat{n} \times \vec{S}_1 \cdot \vec{a}_1 \hat{n} \cdot \vec{v}_1 \log\left(\frac{r}{R_\theta}\right) + 24 \hat{n} \times \vec{S}_1 \cdot \vec{a}_1 \hat{n} \cdot \vec{v}_2 \log\left(\frac{r}{R_\theta}\right) + \frac{1}{\epsilon_d} \left( \frac{8}{3} \vec{S}_1 \times \vec{a}_1 \cdot \vec{v}_2 + \right. \right. \\ \left. \left. \frac{16}{3} \vec{S}_1 \times \vec{v}_1 \cdot \vec{a}_1 - \frac{24}{5} \hat{n} \times \vec{S}_1 \cdot \vec{v}_1 \hat{n} \cdot \vec{a}_1 + \frac{8}{5} \hat{n} \times \vec{S}_1 \cdot \vec{v}_1 \hat{n} \cdot \vec{v}_1 + \frac{56}{5} \hat{n} \times \vec{S}_1 \cdot \vec{a}_1 \hat{n} \cdot \vec{v}_1 - 8 \hat{n} \times \vec{S}_1 \cdot \vec{a}_1 \hat{n} \cdot \vec{v}_2 \right) \right) G^3 + \frac{1}{r^4} \\ m_1^2 m_2 \left( -\frac{688}{49} \hat{n} \times \vec{S}_1 \cdot \vec{v}_1 (\hat{n} \cdot \vec{v}_1)^2 + \frac{96}{7} \hat{n} \times \vec{S}_1 \cdot \vec{v}_1 \log\left(\frac{r}{R_\theta}\right) (\hat{n} \cdot \vec{v}_1)^2 - \frac{96}{25} \vec{S}_1 \times \vec{v}_1 \cdot \vec{v}_2 \hat{n} \cdot \vec{v}_1 + 24 \hat{n} \times \vec{S}_1 \cdot \vec{v}_1 \hat{n} \cdot \vec{v}_2 \hat{n} \cdot \vec{v}_1 + \right. \\ \left. \frac{24}{5} \vec{S}_1 \times \vec{v}_1 \cdot \vec{v}_2 \log\left(\frac{r}{R_\theta}\right) \hat{n} \cdot \vec{v}_1 - 24 \hat{n} \times \vec{S}_1 \cdot \vec{v}_1 \hat{n} \cdot \vec{v}_2 \log\left(\frac{r}{R_\theta}\right) \hat{n} \cdot \vec{v}_1 + \frac{1648 \hat{n} \times \vec{S}_1 \cdot \vec{v}_1 \vec{v}_1 \cdot \vec{v}_1}{1225} - \frac{96}{25} \hat{n} \times \vec{S}_1 \cdot \vec{v}_1 \vec{v}_1 \cdot \vec{v}_2 - \right. \\ \left. \frac{96}{35} \hat{n} \times \vec{S}_1 \cdot \vec{v}_1 \vec{v}_1 \cdot \vec{v}_1 \log\left(\frac{r}{R_\theta}\right) + \frac{24}{5} \hat{n} \times \vec{S}_1 \cdot \vec{v}_1 \vec{v}_1 \cdot \vec{v}_2 \log\left(\frac{r}{R_\theta}\right) + \frac{1}{\epsilon_d} \left( -\frac{32}{7} \hat{n} \times \vec{S}_1 \cdot \vec{v}_1 (\hat{n} \cdot \vec{v}_1)^2 - \right. \right. \\ \left. \left. \frac{8}{5} \vec{S}_1 \times \vec{v}_1 \cdot \vec{v}_2 \hat{n} \cdot \vec{v}_1 + 8 \hat{n} \times \vec{S}_1 \cdot \vec{v}_1 \hat{n} \cdot \vec{v}_2 \hat{n} \cdot \vec{v}_1 + \frac{32}{35} \hat{n} \times \vec{S}_1 \cdot \vec{v}_1 \vec{v}_1 \cdot \vec{v}_1 - \frac{8}{5} \hat{n} \times \vec{S}_1 \cdot \vec{v}_1 \vec{v}_1 \cdot \vec{v}_2 \right) \right) G^3 \Big\}$$

$\{\text{DiagSet}[3, 6, 1],$

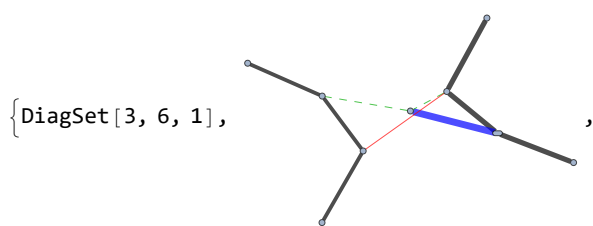

$,$

$$\frac{G^3 m_1 m_2^2 \left( 2 \hat{n} \cdot \vec{v}_1 \vec{S}_1 \times \vec{v}_1 \cdot \vec{v}_2 + 6 \vec{v}_1 \cdot \vec{v}_1 \hat{n} \times \vec{S}_1 \cdot \vec{v}_2 - 8 \vec{v}_1 \cdot \vec{v}_2 \hat{n} \times \vec{S}_1 \cdot \vec{v}_1 \right)}{r^4} \}$$

$\{\text{DiagSet}[3, 6, 2],$

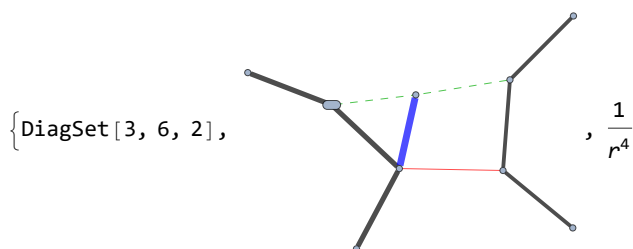

$, \frac{1}{r^4}$

$$G^3 m_1 m_2^2 \left( 72 (\hat{n} \cdot \vec{v}_1)^2 \hat{n} \times \vec{S}_1 \cdot \vec{v}_2 + 24 \hat{n} \cdot \vec{v}_1 \vec{S}_1 \times \vec{v}_1 \cdot \vec{v}_2 - 12 \vec{v}_1 \cdot \vec{v}_1 \hat{n} \times \vec{S}_1 \cdot \vec{v}_2 - 6 \vec{v}_1 \cdot \vec{v}_2 \hat{n} \times \vec{S}_1 \cdot \vec{v}_1 \right) \}$$

$\{\text{DiagSet}[3, 6, 3],$

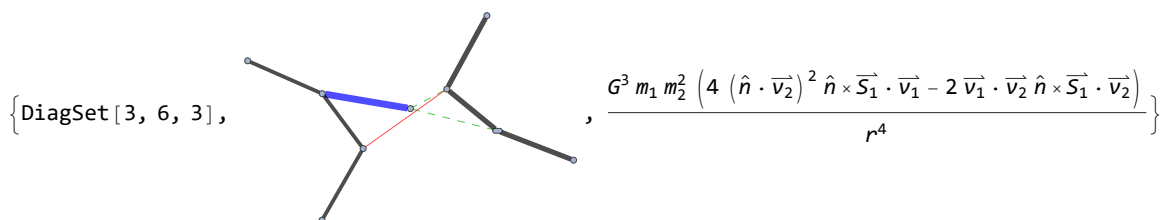

$, \frac{G^3 m_1 m_2^2 \left( 4 (\hat{n} \cdot \vec{v}_2)^2 \hat{n} \times \vec{S}_1 \cdot \vec{v}_1 - 2 \vec{v}_1 \cdot \vec{v}_2 \hat{n} \times \vec{S}_1 \cdot \vec{v}_2 \right)}{r^4} \}$

$\{\text{DiagSet}[3, 6, 4],$

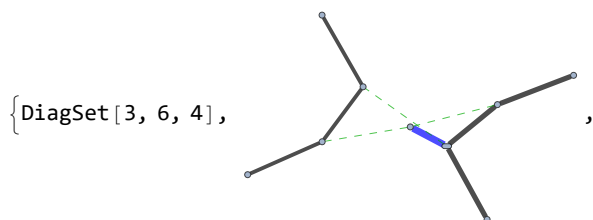

$,$

$$\frac{G^3 m_1 m_2^2 \left( 8 \hat{n} \cdot \vec{v}_2 \vec{S}_1 \times \vec{v}_1 \cdot \vec{v}_2 + 24 \vec{v}_1 \cdot \vec{v}_2 \hat{n} \times \vec{S}_1 \cdot \vec{v}_2 - 8 \vec{v}_2 \cdot \vec{v}_2 \hat{n} \times \vec{S}_1 \cdot \vec{v}_1 \right)}{r^4} \}$$

$\{\text{DiagSet}[3, 6, 5],$

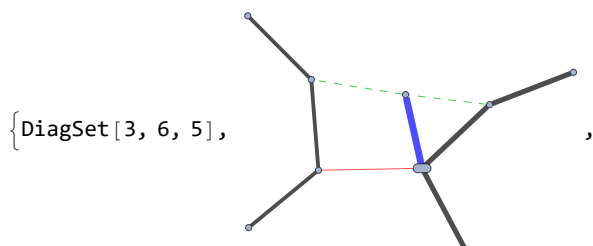

$,$

$$\frac{G^3 m_1 m_2^2 \left( 8 \hat{n} \cdot \vec{v}_1 \vec{S}_1 \times \vec{v}_1 \cdot \vec{v}_2 - 8 \vec{v}_1 \cdot \vec{v}_1 \hat{n} \times \vec{S}_1 \cdot \vec{v}_2 - 40 \vec{v}_1 \cdot \vec{v}_2 \hat{n} \times \vec{S}_1 \cdot \vec{v}_1 \right)}{r^4} \}$$

$\{\text{DiagSet}[3, 6, 6],$ 
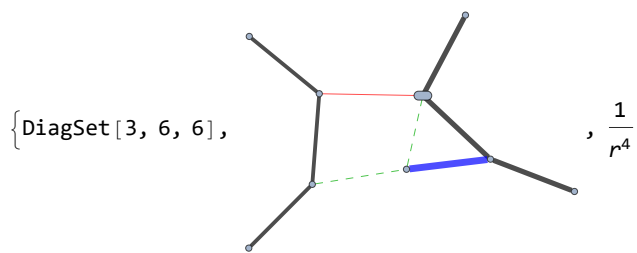
 $, \frac{1}{r^4}$

$$G^3 m_1 m_2^2 \left( -96 (\hat{n} \cdot \vec{v}_1)^2 \hat{n} \times \vec{S}_1 \cdot \vec{v}_2 - 32 \hat{n} \cdot \vec{v}_1 \vec{S}_1 \times \vec{v}_1 \cdot \vec{v}_2 + 16 \vec{v}_1 \cdot \vec{v}_1 \hat{n} \times \vec{S}_1 \cdot \vec{v}_2 + 8 \vec{v}_1 \cdot \vec{v}_2 \hat{n} \times \vec{S}_1 \cdot \vec{v}_1 \right) \}$$

$\{\text{DiagSet}[3, 6, 7],$ 
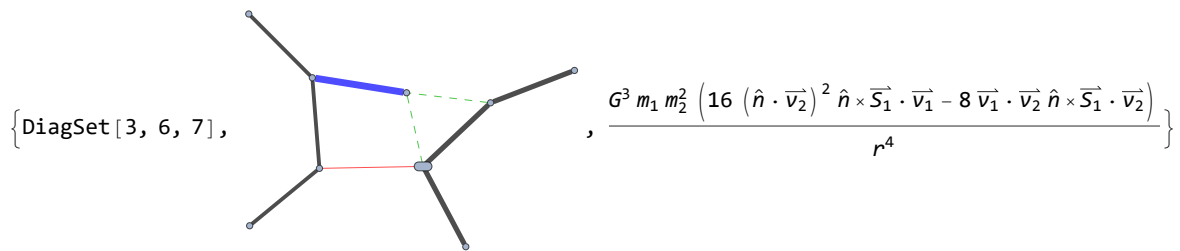
 $, \frac{G^3 m_1 m_2^2 \left( 16 (\hat{n} \cdot \vec{v}_2)^2 \hat{n} \times \vec{S}_1 \cdot \vec{v}_1 - 8 \vec{v}_1 \cdot \vec{v}_2 \hat{n} \times \vec{S}_1 \cdot \vec{v}_2 \right)}{r^4} \}$

$\{\text{DiagSet}[3, 6, 8],$ 
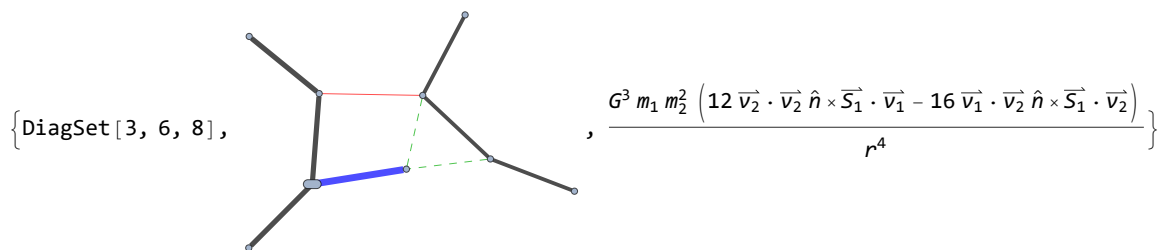
 $, \frac{G^3 m_1 m_2^2 \left( 12 \vec{v}_2 \cdot \vec{v}_2 \hat{n} \times \vec{S}_1 \cdot \vec{v}_1 - 16 \vec{v}_1 \cdot \vec{v}_2 \hat{n} \times \vec{S}_1 \cdot \vec{v}_2 \right)}{r^4} \}$

$\{\text{DiagSet}[3, 6, 9],$ 
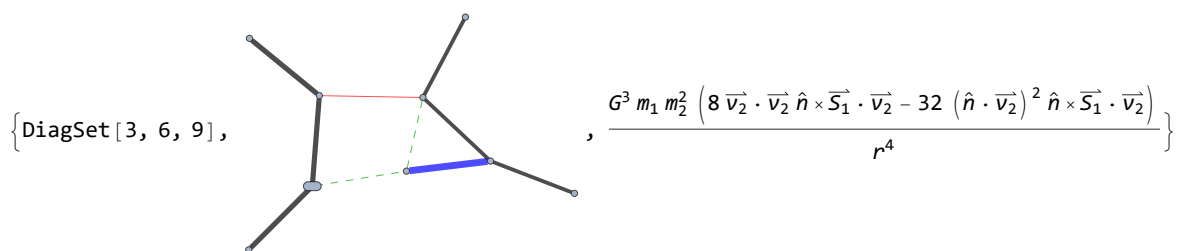
 $, \frac{G^3 m_1 m_2^2 \left( 8 \vec{v}_2 \cdot \vec{v}_2 \hat{n} \times \vec{S}_1 \cdot \vec{v}_2 - 32 (\hat{n} \cdot \vec{v}_2)^2 \hat{n} \times \vec{S}_1 \cdot \vec{v}_2 \right)}{r^4} \}$

$\{\text{DiagSet}[3, 6, 10],$ 
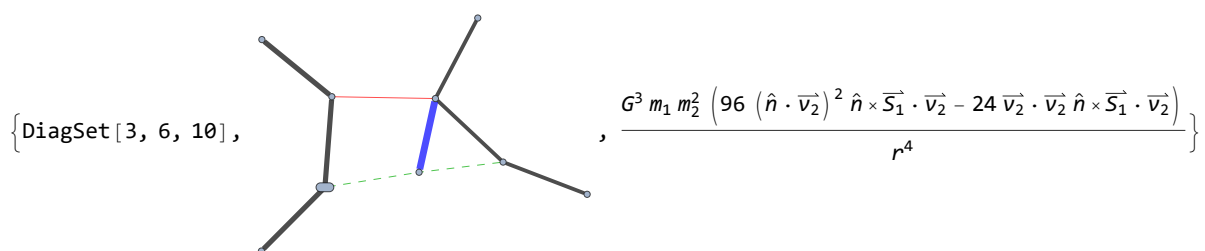
 $, \frac{G^3 m_1 m_2^2 \left( 96 (\hat{n} \cdot \vec{v}_2)^2 \hat{n} \times \vec{S}_1 \cdot \vec{v}_2 - 24 \vec{v}_2 \cdot \vec{v}_2 \hat{n} \times \vec{S}_1 \cdot \vec{v}_2 \right)}{r^4} \}$

$\{\text{DiagSet}[3, 6, 11],$ 
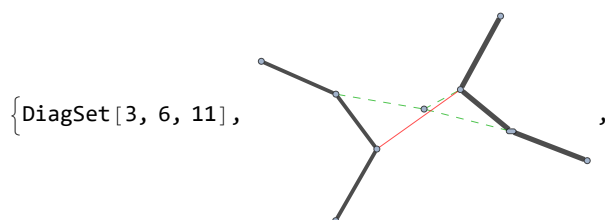
 $,$

$$\frac{1}{r^3} G^3 m_1 m_2^2 \left( 6 \hat{n} \cdot \vec{v}_1 \hat{n} \times \vec{S}_1 \cdot \vec{a}_2 + 6 \hat{n} \cdot \vec{v}_2 \hat{n} \times \vec{S}_1 \cdot \vec{a}_1 - 2 \vec{S}_1 \times \vec{a}_1 \cdot \vec{v}_2 + \right. \\ \left. 2 \vec{S}_1 \times \vec{v}_1 \cdot \vec{a}_2 - 8 \hat{n} \cdot \vec{v}_1 \hat{n} \times \vec{S}_1 \cdot \vec{v}_2 + 2 \hat{n} \cdot \vec{v}_2 \hat{n} \times \vec{S}_1 \cdot \vec{v}_1 - 6 \vec{S}_1 \times \vec{v}_1 \cdot \vec{v}_2 \right) + \frac{1}{r^4}$$

$$G^3 m_1 m_2^2 \left( 24 (\hat{n} \cdot \vec{v}_1)^2 \hat{n} \times \vec{S}_1 \cdot \vec{v}_2 + 14 \hat{n} \cdot \vec{v}_1 \vec{S}_1 \times \vec{v}_1 \cdot \vec{v}_2 - 14 \hat{n} \cdot \vec{v}_2 \hat{n} \cdot \vec{v}_1 \hat{n} \times \vec{S}_1 \cdot \vec{v}_1 + 24 \hat{n} \cdot \vec{v}_2 \hat{n} \cdot \vec{v}_1 \hat{n} \times \vec{S}_1 \cdot \vec{v}_2 + \right. \\ \left. 6 (\hat{n} \cdot \vec{v}_2)^2 \hat{n} \times \vec{S}_1 \cdot \vec{v}_1 + 2 \hat{n} \cdot \vec{v}_2 \vec{S}_1 \times \vec{v}_1 \cdot \vec{v}_2 - 6 \vec{v}_1 \cdot \vec{v}_1 \hat{n} \times \vec{S}_1 \cdot \vec{v}_2 + 6 \vec{v}_1 \cdot \vec{v}_2 \hat{n} \times \vec{S}_1 \cdot \vec{v}_1 - 6 \vec{v}_1 \cdot \vec{v}_2 \hat{n} \times \vec{S}_1 \cdot \vec{v}_2 \right) \}$$

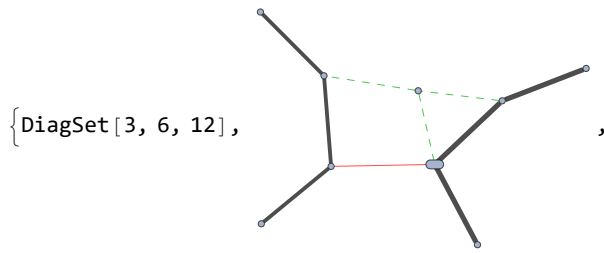

$$\frac{1}{r^3} G^3 m_1 m_2^2 \left( 24 \hat{n} \cdot \vec{v}_1 \hat{n} \times \vec{S}_1 \cdot \vec{a}_2 + 24 \hat{n} \cdot \vec{v}_2 \hat{n} \times \vec{S}_1 \cdot \vec{a}_1 - 8 \vec{S}_1 \times \vec{a}_1 \cdot \vec{v}_2 + \right. \\ \left. 8 \vec{S}_1 \times \vec{v}_1 \cdot \vec{a}_2 - 32 \hat{n} \cdot \vec{v}_1 \hat{n} \times \vec{S}_1 \cdot \vec{v}_2 + 8 \hat{n} \cdot \vec{v}_2 \hat{n} \times \vec{S}_1 \cdot \vec{v}_1 - 24 \vec{S}_1 \times \vec{v}_1 \cdot \vec{v}_2 \right) + \frac{1}{r^4} \\ G^3 m_1 m_2^2 \left( 128 (\hat{n} \cdot \vec{v}_1)^2 \hat{n} \times \vec{S}_1 \cdot \vec{v}_2 + 72 \hat{n} \cdot \vec{v}_1 \vec{S}_1 \times \vec{v}_1 \cdot \vec{v}_2 - 40 \hat{n} \cdot \vec{v}_2 \hat{n} \cdot \vec{v}_1 \hat{n} \times \vec{S}_1 \cdot \vec{v}_1 + 64 \hat{n} \cdot \vec{v}_2 \hat{n} \cdot \vec{v}_1 \hat{n} \times \vec{S}_1 \cdot \vec{v}_2 + \right. \\ \left. 8 (\hat{n} \cdot \vec{v}_2)^2 \hat{n} \times \vec{S}_1 \cdot \vec{v}_1 - 8 \hat{n} \cdot \vec{v}_2 \vec{S}_1 \times \vec{v}_1 \cdot \vec{v}_2 - 24 \vec{v}_1 \cdot \vec{v}_1 \hat{n} \times \vec{S}_1 \cdot \vec{v}_2 + 24 \vec{v}_1 \cdot \vec{v}_2 \hat{n} \times \vec{S}_1 \cdot \vec{v}_1 - 24 \vec{v}_1 \cdot \vec{v}_2 \hat{n} \times \vec{S}_1 \cdot \vec{v}_2 \right) \}$$

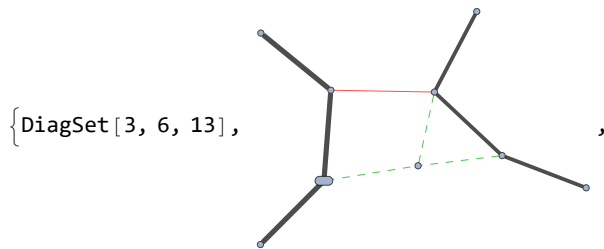

$$\frac{G^3 m_1 m_2^2 \left( -32 \hat{n} \cdot \vec{v}_2 \hat{n} \times \vec{a}_2 \cdot \vec{S}_1 + 16 \vec{a}_2 \times \vec{S}_1 \cdot \vec{v}_2 - 16 \hat{n} \cdot \vec{v}_2 \hat{n} \times \vec{S}_1 \cdot \vec{v}_2 \right)}{r^3} + \frac{1}{r^4} G^3 m_1 m_2^2 \\ \left( 80 (\hat{n} \cdot \vec{v}_2)^2 \hat{n} \times \vec{S}_1 \cdot \vec{v}_2 + 16 \hat{n} \cdot \vec{v}_2 \vec{S}_1 \times \vec{v}_1 \cdot \vec{v}_2 + 48 \hat{n} \cdot \vec{v}_1 \hat{n} \cdot \vec{v}_2 \hat{n} \times \vec{S}_1 \cdot \vec{v}_2 - 16 \vec{v}_1 \cdot \vec{v}_2 \hat{n} \times \vec{S}_1 \cdot \vec{v}_2 - 12 \vec{v}_2 \cdot \vec{v}_2 \hat{n} \times \vec{S}_1 \cdot \vec{v}_2 \right) \}$$

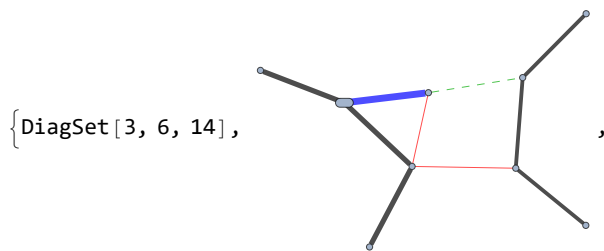

$$\frac{G^3 m_1 m_2^2 \left( -2 \hat{n} \cdot \vec{v}_1 \hat{n} \times \vec{S}_1 \cdot \vec{a}_2 - 2 \vec{S}_1 \times \vec{v}_1 \cdot \vec{a}_2 \right)}{r^3} + \frac{1}{r^4} G^3 m_1 m_2^2 \left( 16 (\hat{n} \cdot \vec{v}_1)^2 \hat{n} \times \vec{S}_1 \cdot \vec{v}_2 + 10 \hat{n} \cdot \vec{v}_1 \vec{S}_1 \times \vec{v}_1 \cdot \vec{v}_2 - \right. \\ \left. 16 \hat{n} \cdot \vec{v}_2 \hat{n} \cdot \vec{v}_1 \hat{n} \times \vec{S}_1 \cdot \vec{v}_2 - 8 \hat{n} \cdot \vec{v}_2 \vec{S}_1 \times \vec{v}_1 \cdot \vec{v}_2 - 2 \vec{v}_1 \cdot \vec{v}_1 \hat{n} \times \vec{S}_1 \cdot \vec{v}_2 + 2 \vec{v}_1 \cdot \vec{v}_2 \hat{n} \times \vec{S}_1 \cdot \vec{v}_1 + 2 \vec{v}_1 \cdot \vec{v}_2 \hat{n} \times \vec{S}_1 \cdot \vec{v}_2 \right) \}$$

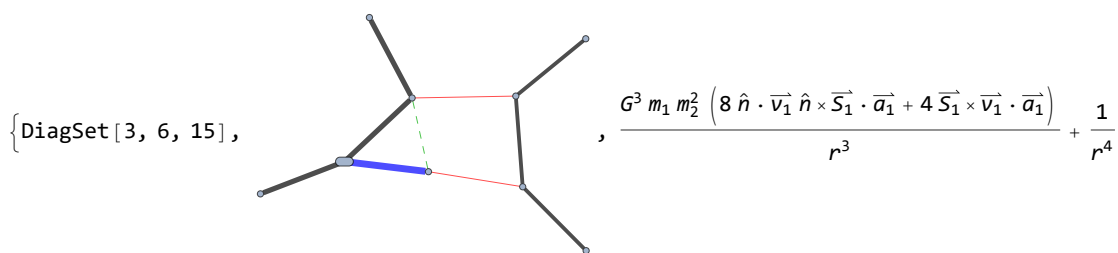

$$G^3 m_1 m_2^2 \left( -16 (\hat{n} \cdot \vec{v}_1)^2 \hat{n} \times \vec{S}_1 \cdot \vec{v}_1 - 2 \hat{n} \cdot \vec{v}_1 \vec{S}_1 \times \vec{v}_1 \cdot \vec{v}_2 + 16 \hat{n} \cdot \vec{v}_2 \hat{n} \cdot \vec{v}_1 \hat{n} \times \vec{S}_1 \cdot \vec{v}_1 - 2 \vec{v}_1 \cdot \vec{v}_2 \hat{n} \times \vec{S}_1 \cdot \vec{v}_1 \right) \Bigg\}$$

{DiagSet[3, 6, 16],

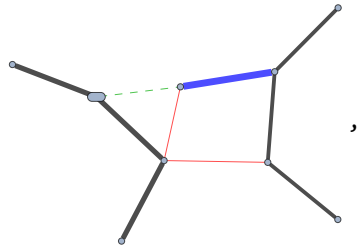

$$\frac{G^3 m_1 m_2^2 \left( 6 (\hat{n} \cdot \vec{v}_2)^2 \hat{n} \times \vec{S}_1 \cdot \vec{v}_2 - 2 \hat{n} \cdot \vec{v}_2 \vec{S}_1 \times \vec{v}_1 \cdot \vec{v}_2 - 6 \hat{n} \cdot \vec{v}_1 \hat{n} \cdot \vec{v}_2 \hat{n} \times \vec{S}_1 \cdot \vec{v}_2 \right)}{r^4} - \frac{2 G^3 m_1 m_2^2 \hat{n} \cdot \vec{v}_2 \hat{n} \times \vec{S}_1 \cdot \vec{v}_2}{r^3} \Bigg\}$$

{DiagSet[3, 6, 17],

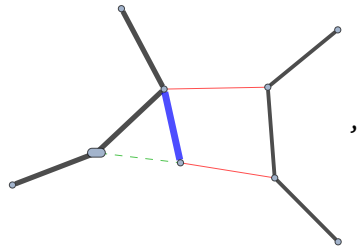

$$\frac{1}{r^4} G^3 m_1 m_2^2 \left( 72 (\hat{n} \cdot \vec{v}_1)^2 \hat{n} \times \vec{S}_1 \cdot \vec{v}_1 + 18 \hat{n} \cdot \vec{v}_1 \vec{S}_1 \times \vec{v}_1 \cdot \vec{v}_2 - 72 \hat{n} \cdot \vec{v}_2 \hat{n} \cdot \vec{v}_1 \hat{n} \times \vec{S}_1 \cdot \vec{v}_1 - \right. \\ \left. 18 \vec{v}_1 \cdot \vec{v}_1 \hat{n} \times \vec{S}_1 \cdot \vec{v}_1 + 18 \vec{v}_1 \cdot \vec{v}_2 \hat{n} \times \vec{S}_1 \cdot \vec{v}_1 \right) - \frac{24 G^3 m_1 m_2^2 \hat{n} \cdot \vec{v}_1 \hat{n} \times \vec{S}_1 \cdot \vec{v}_1}{r^3} \Bigg\}$$

{DiagSet[3, 6, 18],

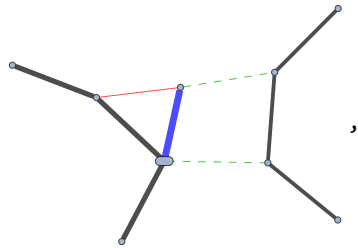

$$\frac{G^3 m_1 m_2^2 \left( 8 \hat{n} \cdot \vec{a}_2 \hat{n} \times \vec{S}_1 \cdot \vec{v}_2 + 8 \hat{n} \cdot \vec{v}_2 \hat{n} \times \vec{S}_1 \cdot \vec{a}_2 + 8 \vec{S}_1 \times \vec{v}_2 \cdot \vec{a}_2 \right)}{r^3} + \frac{1}{r^4} G^3 m_1 m_2^2 \left( 32 (\hat{n} \cdot \vec{v}_2)^2 \hat{n} \times \vec{S}_1 \cdot \vec{v}_2 - \right. \\ \left. 8 \hat{n} \cdot \vec{v}_2 \vec{S}_1 \times \vec{v}_1 \cdot \vec{v}_2 - 32 \hat{n} \cdot \vec{v}_1 \hat{n} \cdot \vec{v}_2 \hat{n} \times \vec{S}_1 \cdot \vec{v}_2 + 8 \vec{v}_1 \cdot \vec{v}_2 \hat{n} \times \vec{S}_1 \cdot \vec{v}_2 + 8 \vec{v}_2 \cdot \vec{v}_2 \hat{n} \times \vec{S}_1 \cdot \vec{v}_1 - 16 \vec{v}_2 \cdot \vec{v}_2 \hat{n} \times \vec{S}_1 \cdot \vec{v}_2 \right) \Bigg\}$$

{DiagSet[3, 6, 19],

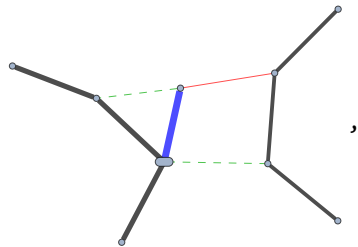

$$\frac{G^3 m_1 m_2^2 \left( -16 \hat{n} \cdot \vec{a}_1 \hat{n} \times \vec{S}_1 \cdot \vec{v}_2 - 16 \hat{n} \cdot \vec{v}_2 \hat{n} \times \vec{S}_1 \cdot \vec{a}_1 + 16 \vec{S}_1 \times \vec{a}_1 \cdot \vec{v}_2 \right)}{r^3} + \frac{1}{r^4} \\ G^3 m_1 m_2^2 \left( 16 (\hat{n} \cdot \vec{v}_1)^2 \hat{n} \times \vec{S}_1 \cdot \vec{v}_2 + 16 \hat{n} \cdot \vec{v}_2 \hat{n} \cdot \vec{v}_1 \hat{n} \times \vec{S}_1 \cdot \vec{v}_1 - 16 \hat{n} \cdot \vec{v}_2 \hat{n} \cdot \vec{v}_1 \hat{n} \times \vec{S}_1 \cdot \vec{v}_2 - \right. \\ \left. 16 (\hat{n} \cdot \vec{v}_2)^2 \hat{n} \times \vec{S}_1 \cdot \vec{v}_1 + 8 \hat{n} \cdot \vec{v}_2 \vec{S}_1 \times \vec{v}_1 \cdot \vec{v}_2 - 16 \vec{v}_1 \cdot \vec{v}_2 \hat{n} \times \vec{S}_1 \cdot \vec{v}_1 + 8 \vec{v}_1 \cdot \vec{v}_2 \hat{n} \times \vec{S}_1 \cdot \vec{v}_2 + 8 \vec{v}_2 \cdot \vec{v}_2 \hat{n} \times \vec{S}_1 \cdot \vec{v}_1 \right) \Bigg\}$$



{DiagSet[3, 6, 20],

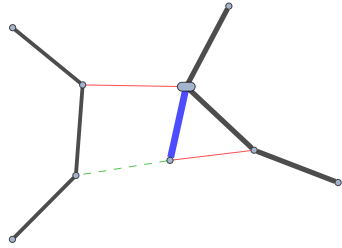

,

$$\frac{G^3 m_1 m_2^2 \left( -8 \hat{n} \cdot \vec{a}_2 \hat{n} \times \vec{S}_1 \cdot \vec{v}_1 + 8 \hat{n} \cdot \vec{v}_1 \hat{n} \times \vec{S}_1 \cdot \vec{a}_2 - 8 \vec{S}_1 \times \vec{v}_1 \cdot \vec{a}_2 \right)}{r^3} + \frac{1}{r^4}$$

$$G^3 m_1 m_2^2 \left( -16 \left( \hat{n} \cdot \vec{v}_1 \right)^2 \hat{n} \times \vec{S}_1 \cdot \vec{v}_2 + 8 \hat{n} \cdot \vec{v}_1 \vec{S}_1 \times \vec{v}_1 \cdot \vec{v}_2 + 16 \hat{n} \cdot \vec{v}_2 \hat{n} \cdot \vec{v}_1 \hat{n} \times \vec{S}_1 \cdot \vec{v}_1 + 16 \hat{n} \cdot \vec{v}_2 \hat{n} \cdot \vec{v}_1 \hat{n} \times \vec{S}_1 \cdot \vec{v}_2 - \right.$$

$$\left. 16 \left( \hat{n} \cdot \vec{v}_2 \right)^2 \hat{n} \times \vec{S}_1 \cdot \vec{v}_1 + 8 \vec{v}_1 \cdot \vec{v}_1 \hat{n} \times \vec{S}_1 \cdot \vec{v}_2 + 8 \vec{v}_1 \cdot \vec{v}_2 \hat{n} \times \vec{S}_1 \cdot \vec{v}_1 - 16 \vec{v}_1 \cdot \vec{v}_2 \hat{n} \times \vec{S}_1 \cdot \vec{v}_2 \right) \}$$

{DiagSet[3, 6, 21],

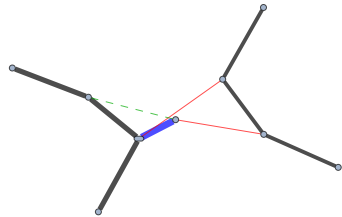

,

$$\frac{G^3 m_1 m_2^2 \left( 16 \hat{n} \cdot \vec{a}_1 \hat{n} \times \vec{S}_1 \cdot \vec{v}_1 - 16 \hat{n} \cdot \vec{v}_1 \hat{n} \times \vec{S}_1 \cdot \vec{a}_1 + 16 \vec{S}_1 \times \vec{v}_1 \cdot \vec{a}_1 \right)}{r^3} + \frac{1}{r^4}$$

$$G^3 m_1 m_2^2 \left( -8 \hat{n} \cdot \vec{v}_1 \vec{S}_1 \times \vec{v}_1 \cdot \vec{v}_2 - 16 \vec{v}_1 \cdot \vec{v}_1 \hat{n} \times \vec{S}_1 \cdot \vec{v}_1 + 8 \vec{v}_1 \cdot \vec{v}_1 \hat{n} \times \vec{S}_1 \cdot \vec{v}_2 + 8 \vec{v}_1 \cdot \vec{v}_2 \hat{n} \times \vec{S}_1 \cdot \vec{v}_1 \right) \}$$

{DiagSet[3, 6, 22],

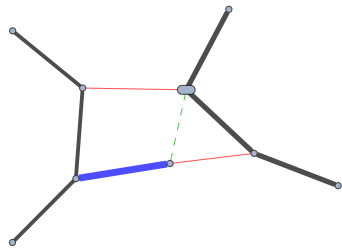

,

$$\frac{G^3 m_1 m_2^2 \left( -8 \left( \hat{n} \cdot \vec{v}_2 \right)^2 \hat{n} \times \vec{S}_1 \cdot \vec{v}_2 - 8 \hat{n} \cdot \vec{v}_2 \vec{S}_1 \times \vec{v}_1 \cdot \vec{v}_2 + 8 \hat{n} \cdot \vec{v}_1 \hat{n} \cdot \vec{v}_2 \hat{n} \times \vec{S}_1 \cdot \vec{v}_2 \right)}{r^4} - \frac{8 G^3 m_1 m_2^2 \hat{n} \cdot \vec{v}_2 \hat{n} \times \vec{S}_1 \cdot \vec{v}_2}{r^3} \}$$

{DiagSet[3, 6, 23],

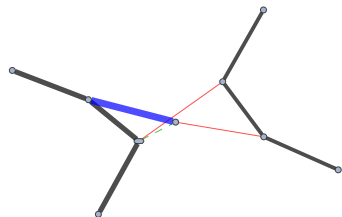

,

$$\frac{1}{r^4} G^3 m_1 m_2^2 \left( -128 \left( \hat{n} \cdot \vec{v}_1 \right)^2 \hat{n} \times \vec{S}_1 \cdot \vec{v}_1 - 24 \hat{n} \cdot \vec{v}_1 \vec{S}_1 \times \vec{v}_1 \cdot \vec{v}_2 + 128 \hat{n} \cdot \vec{v}_2 \hat{n} \cdot \vec{v}_1 \hat{n} \times \vec{S}_1 \cdot \vec{v}_1 + \right.$$

$$\left. 24 \vec{v}_1 \cdot \vec{v}_1 \hat{n} \times \vec{S}_1 \cdot \vec{v}_1 - 24 \vec{v}_1 \cdot \vec{v}_2 \hat{n} \times \vec{S}_1 \cdot \vec{v}_1 \right) + \frac{32 G^3 m_1 m_2^2 \hat{n} \cdot \vec{v}_1 \hat{n} \times \vec{S}_1 \cdot \vec{v}_1}{r^3} \}$$

$\{\text{DiagSet}[3, 6, 24],$ 
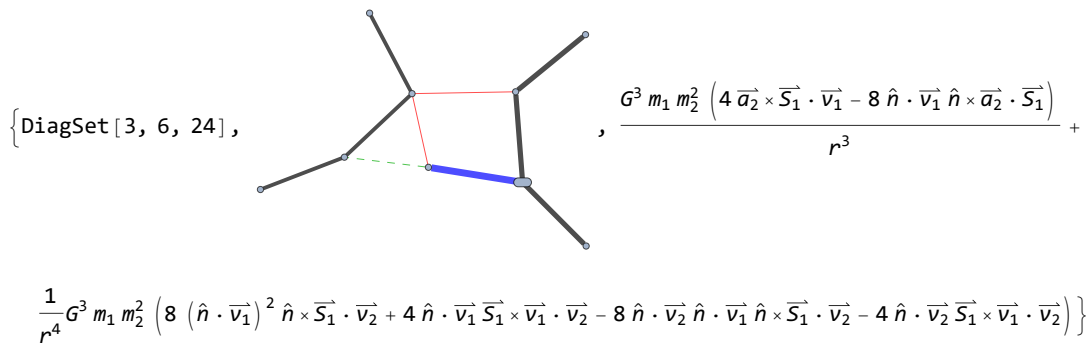
 $, \frac{G^3 m_1 m_2^2 \left( 4 \vec{a}_2 \times \vec{S}_1 \cdot \vec{v}_1 - 8 \hat{n} \cdot \vec{v}_1 \hat{n} \times \vec{a}_2 \cdot \vec{S}_1 \right)}{r^3} +$ 
 $\frac{1}{r^4} G^3 m_1 m_2^2 \left( 8 \left( \hat{n} \cdot \vec{v}_1 \right)^2 \hat{n} \times \vec{S}_1 \cdot \vec{v}_2 + 4 \hat{n} \cdot \vec{v}_1 \vec{S}_1 \times \vec{v}_1 \cdot \vec{v}_2 - 8 \hat{n} \cdot \vec{v}_2 \hat{n} \cdot \vec{v}_1 \hat{n} \times \vec{S}_1 \cdot \vec{v}_2 - 4 \hat{n} \cdot \vec{v}_2 \vec{S}_1 \times \vec{v}_1 \cdot \vec{v}_2 \right) \}$

$\{\text{DiagSet}[3, 6, 25],$ 
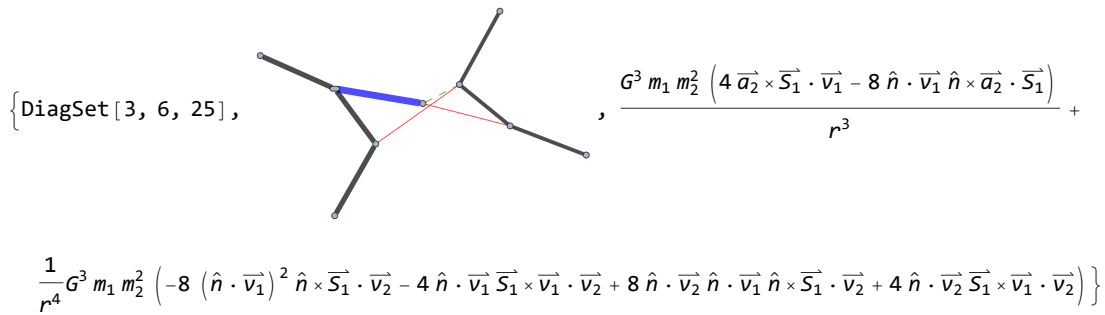
 $, \frac{G^3 m_1 m_2^2 \left( 4 \vec{a}_2 \times \vec{S}_1 \cdot \vec{v}_1 - 8 \hat{n} \cdot \vec{v}_1 \hat{n} \times \vec{a}_2 \cdot \vec{S}_1 \right)}{r^3} +$ 
 $\frac{1}{r^4} G^3 m_1 m_2^2 \left( -8 \left( \hat{n} \cdot \vec{v}_1 \right)^2 \hat{n} \times \vec{S}_1 \cdot \vec{v}_2 - 4 \hat{n} \cdot \vec{v}_1 \vec{S}_1 \times \vec{v}_1 \cdot \vec{v}_2 + 8 \hat{n} \cdot \vec{v}_2 \hat{n} \cdot \vec{v}_1 \hat{n} \times \vec{S}_1 \cdot \vec{v}_2 + 4 \hat{n} \cdot \vec{v}_2 \vec{S}_1 \times \vec{v}_1 \cdot \vec{v}_2 \right) \}$

$\{\text{DiagSet}[3, 6, 26],$ 
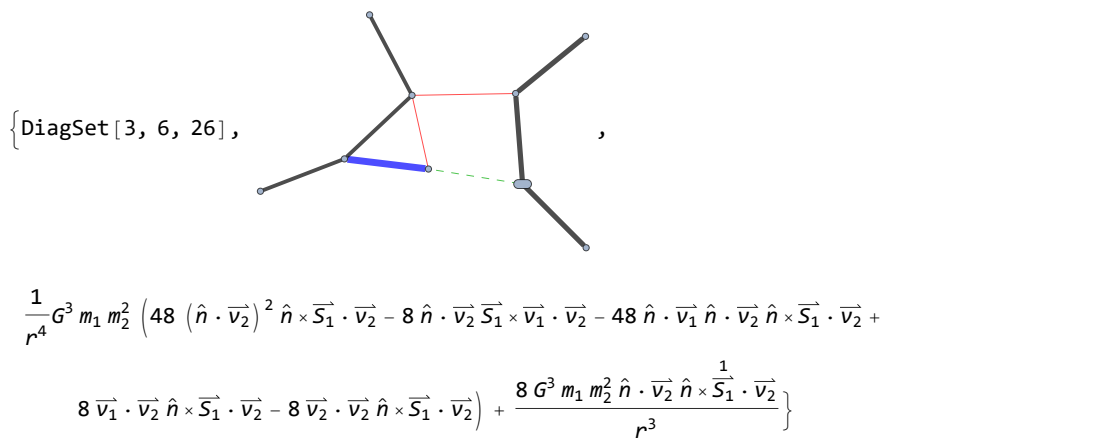
 $, \frac{1}{r^4} G^3 m_1 m_2^2 \left( 48 \left( \hat{n} \cdot \vec{v}_2 \right)^2 \hat{n} \times \vec{S}_1 \cdot \vec{v}_2 - 8 \hat{n} \cdot \vec{v}_2 \vec{S}_1 \times \vec{v}_1 \cdot \vec{v}_2 - 48 \hat{n} \cdot \vec{v}_1 \hat{n} \cdot \vec{v}_2 \hat{n} \times \vec{S}_1 \cdot \vec{v}_2 + \right.$ 
 $\left. 8 \vec{v}_1 \cdot \vec{v}_2 \hat{n} \times \vec{S}_1 \cdot \vec{v}_2 - 8 \vec{v}_2 \cdot \vec{v}_2 \hat{n} \times \vec{S}_1 \cdot \vec{v}_2 \right) + \frac{8 G^3 m_1 m_2^2 \hat{n} \cdot \vec{v}_2 \hat{n} \times \vec{S}_1 \cdot \vec{v}_2}{r^3} \}$

$\{\text{DiagSet}[3, 6, 27],$ 
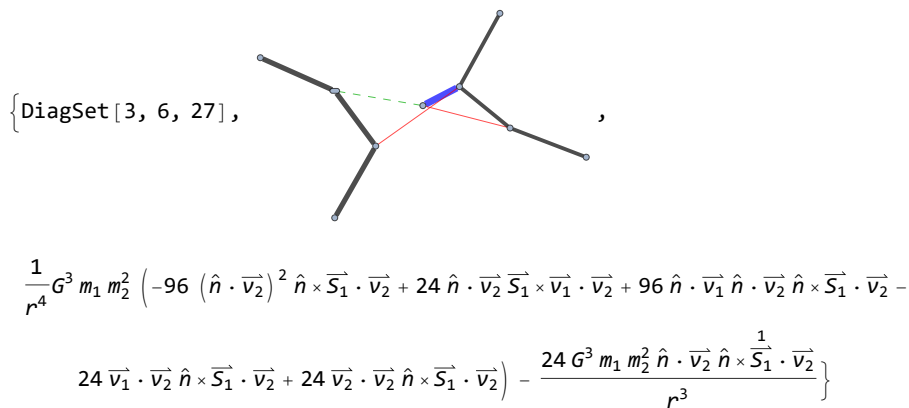
 $, \frac{1}{r^4} G^3 m_1 m_2^2 \left( -96 \left( \hat{n} \cdot \vec{v}_2 \right)^2 \hat{n} \times \vec{S}_1 \cdot \vec{v}_2 + 24 \hat{n} \cdot \vec{v}_2 \vec{S}_1 \times \vec{v}_1 \cdot \vec{v}_2 + 96 \hat{n} \cdot \vec{v}_1 \hat{n} \cdot \vec{v}_2 \hat{n} \times \vec{S}_1 \cdot \vec{v}_2 - \right.$ 
 $\left. 24 \vec{v}_1 \cdot \vec{v}_2 \hat{n} \times \vec{S}_1 \cdot \vec{v}_2 + 24 \vec{v}_2 \cdot \vec{v}_2 \hat{n} \times \vec{S}_1 \cdot \vec{v}_2 \right) - \frac{24 G^3 m_1 m_2^2 \hat{n} \cdot \vec{v}_2 \hat{n} \times \vec{S}_1 \cdot \vec{v}_2}{r^3} \}$

$\{\text{DiagSet}[3, 6, 28],$ 
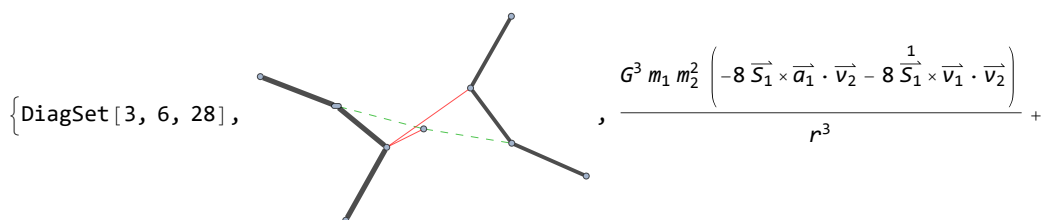
 $, \frac{G^3 m_1 m_2^2 \left( -8 \vec{S}_1 \times \vec{a}_1 \cdot \vec{v}_2 - 8 \vec{S}_1 \times \vec{v}_1 \cdot \vec{v}_2 \right)}{r^3} +$

$$\frac{1}{r^4} G^3 m_1 m_2^2 \left( 5 \hat{n} \cdot \vec{v}_1 \vec{S}_1 \times \vec{v}_1 \cdot \vec{v}_2 - 9 \vec{v}_1 \cdot \vec{v}_1 \hat{n} \times \vec{S}_1 \cdot \vec{v}_2 + 7 \vec{v}_1 \cdot \vec{v}_2 \hat{n} \times \vec{S}_1 \cdot \vec{v}_1 + 4 \vec{v}_2 \cdot \vec{v}_2 \hat{n} \times \vec{S}_1 \cdot \vec{v}_2 \right) \Big\}$$

{DiagSet[3, 6, 29], 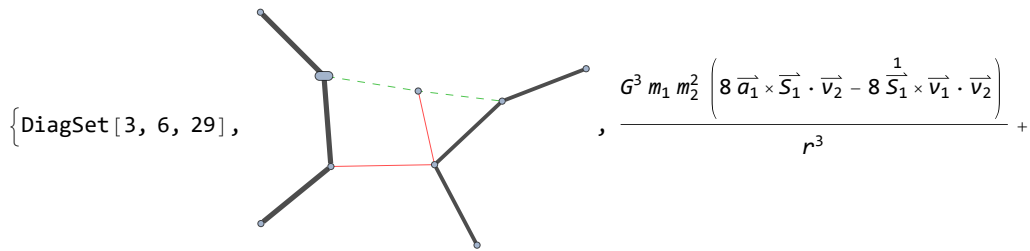

$$, \frac{G^3 m_1 m_2^2 \left( 8 \vec{a}_1 \times \vec{S}_1 \cdot \vec{v}_2 - 8 \vec{S}_1 \times \vec{v}_1 \cdot \vec{v}_2 \right)}{r^3} +$$

$$\frac{1}{r^4} G^3 m_1 m_2^2 \left( 4 \hat{n} \cdot \vec{v}_1 \vec{S}_1 \times \vec{v}_1 \cdot \vec{v}_2 + 12 \vec{v}_1 \cdot \vec{v}_1 \hat{n} \times \vec{S}_1 \cdot \vec{v}_2 + 12 \vec{v}_1 \cdot \vec{v}_2 \hat{n} \times \vec{S}_1 \cdot \vec{v}_1 - 32 \vec{v}_2 \cdot \vec{v}_2 \hat{n} \times \vec{S}_1 \cdot \vec{v}_2 \right) \Big\}$$

{DiagSet[3, 6, 30], 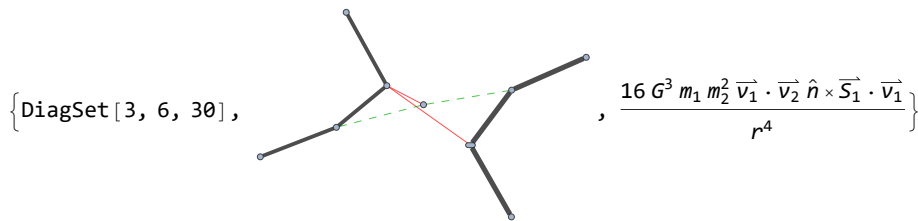

$$, \frac{16 G^3 m_1 m_2^2 \vec{v}_1 \cdot \vec{v}_2 \hat{n} \times \vec{S}_1 \cdot \vec{v}_1}{r^4} \Big\}$$

{DiagSet[3, 6, 31], 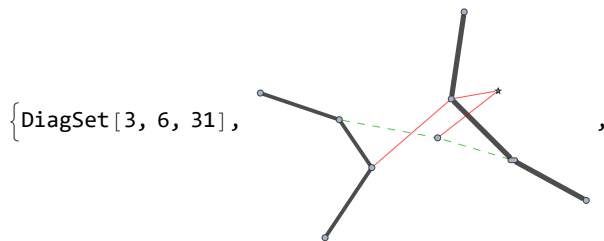

$$,$$

$$\frac{1}{r^3} G^3 m_1 m_2^2 \left( 3 \hat{n} \cdot \vec{a}_2 \hat{n} \times \vec{S}_1 \cdot \vec{v}_1 - 2 \hat{n} \cdot \vec{v}_2 \hat{n} \times \vec{S}_1 \cdot \vec{a}_2 - \vec{S}_1 \times \vec{v}_1 \cdot \vec{a}_2 + 3 \hat{n} \cdot \vec{v}_2 \hat{n} \times \vec{S}_1 \cdot \vec{v}_1 - 2 \hat{n} \cdot \vec{v}_2 \hat{n} \times \vec{S}_1 \cdot \vec{v}_2 - \left( \vec{S}_1 \times \vec{v}_1 \cdot \vec{v}_2 \right) \right) +$$

$$\frac{1}{r^4} G^3 m_1 m_2^2 \left( 9 \left( \hat{n} \cdot \vec{v}_2 \right)^2 \hat{n} \times \vec{S}_1 \cdot \vec{v}_1 - 4 \left( \hat{n} \cdot \vec{v}_2 \right)^2 \hat{n} \times \vec{S}_1 \cdot \vec{v}_2 - 2 \hat{n} \cdot \vec{v}_2 \vec{S}_1 \times \vec{v}_1 \cdot \vec{v}_2 - 5 \hat{n} \cdot \vec{v}_1 \hat{n} \cdot \vec{v}_2 \hat{n} \times \vec{S}_1 \cdot \vec{v}_1 + \right.$$

$$\left. 2 \hat{n} \cdot \vec{v}_1 \hat{n} \cdot \vec{v}_2 \hat{n} \times \vec{S}_1 \cdot \vec{v}_2 + \hat{n} \cdot \vec{v}_1 \vec{S}_1 \times \vec{v}_1 \cdot \vec{v}_2 + \vec{v}_1 \cdot \vec{v}_2 \hat{n} \times \vec{S}_1 \cdot \vec{v}_1 + 2 \vec{v}_1 \cdot \vec{v}_2 \hat{n} \times \vec{S}_1 \cdot \vec{v}_2 - 3 \vec{v}_2 \cdot \vec{v}_2 \hat{n} \times \vec{S}_1 \cdot \vec{v}_1 \right) \Big\}$$

{DiagSet[3, 6, 32], 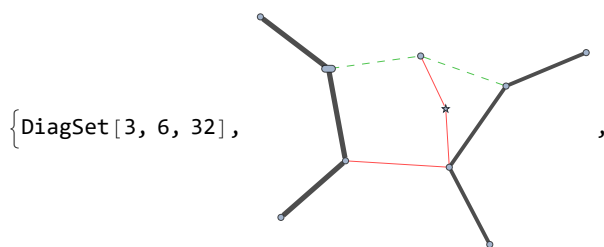

$$,$$

$$\frac{1}{r^3} G^3 m_1 m_2^2 \left( 4 \hat{n} \cdot \vec{a}_2 \hat{n} \times \vec{S}_1 \cdot \vec{v}_2 - 4 \hat{n} \cdot \vec{v}_1 \hat{n} \times \vec{a}_2 \cdot \vec{S}_1 + 4 \hat{n} \cdot \vec{v}_2 \hat{n} \times \vec{a}_2 \cdot \vec{S}_1 - 2 \vec{a}_2 \times \vec{S}_1 \cdot \vec{v}_2 + 4 \hat{n} \cdot \vec{v}_1 \hat{n} \times \vec{S}_1 \cdot \vec{v}_2 \right) +$$

$$\frac{1}{r^4} G^3 m_1 m_2^2 \left( -8 \left( \hat{n} \cdot \vec{v}_1 \right)^2 \hat{n} \times \vec{S}_1 \cdot \vec{v}_2 - 4 \hat{n} \cdot \vec{v}_1 \vec{S}_1 \times \vec{v}_1 \cdot \vec{v}_2 + 4 \hat{n} \cdot \vec{v}_2 \hat{n} \cdot \vec{v}_1 \hat{n} \times \vec{S}_1 \cdot \vec{v}_2 + 4 \vec{v}_1 \cdot \vec{v}_2 \hat{n} \times \vec{S}_1 \cdot \vec{v}_2 \right) \Big\}$$

$\{\text{DiagSet}[3, 6, 33],$ 
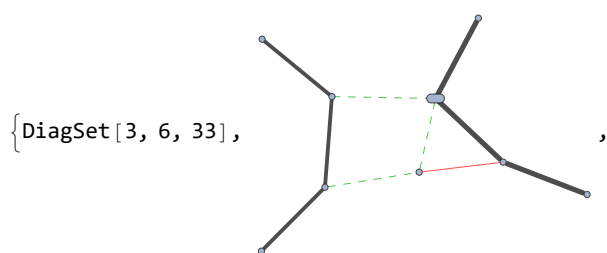
 $,$

$$\frac{32 G^3 m_1 m_2^2 \vec{S}_1 \times \vec{v}_2 \cdot \vec{a}_2}{r^3} + \frac{G^3 m_1 m_2^2 \left( 8 \hat{n} \cdot \vec{v}_2 \vec{S}_1 \times \vec{v}_1 \cdot \vec{v}_2 - 16 \vec{v}_1 \cdot \vec{v}_2 \hat{n} \times \vec{S}_1 \cdot \vec{v}_2 \right)}{r^4} \}$$

$\{\text{DiagSet}[3, 6, 34],$ 
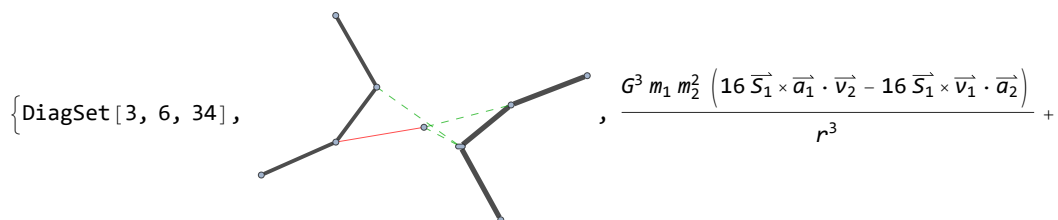
 $,$ 
 $\frac{G^3 m_1 m_2^2 \left( 16 \vec{S}_1 \times \vec{a}_1 \cdot \vec{v}_2 - 16 \vec{S}_1 \times \vec{v}_1 \cdot \vec{a}_2 \right)}{r^3} +$

$$\frac{1}{r^4} G^3 m_1 m_2^2 \left( -24 \hat{n} \cdot \vec{v}_1 \vec{S}_1 \times \vec{v}_1 \cdot \vec{v}_2 + 16 \hat{n} \cdot \vec{v}_2 \vec{S}_1 \times \vec{v}_1 \cdot \vec{v}_2 + 8 \vec{v}_1 \cdot \vec{v}_1 \hat{n} \times \vec{S}_1 \cdot \vec{v}_2 + 8 \vec{v}_1 \cdot \vec{v}_2 \hat{n} \times \vec{S}_1 \cdot \vec{v}_1 \right) \}$$

$\{\text{DiagSet}[3, 6, 35],$ 
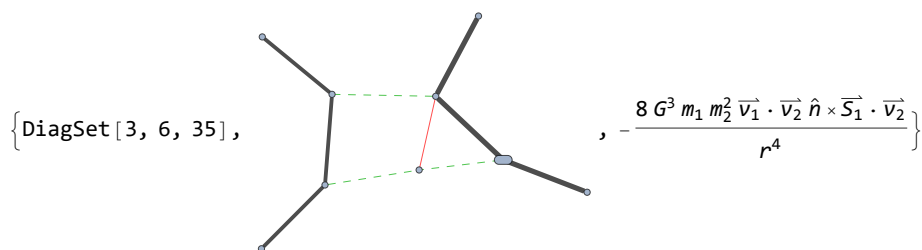
 $,$ 
 $-\frac{8 G^3 m_1 m_2^2 \vec{v}_1 \cdot \vec{v}_2 \hat{n} \times \vec{S}_1 \cdot \vec{v}_2}{r^4} \}$

$\{\text{DiagSet}[3, 6, 36],$ 
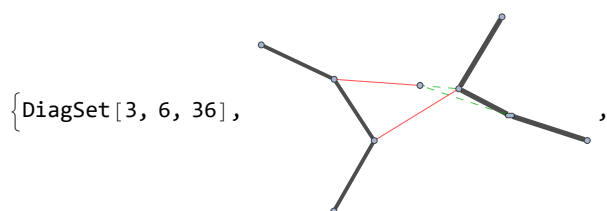
 $,$

$$\frac{G^3 m_1 m_2^2 \left( -4 \vec{v}_1 \cdot \vec{v}_1 \hat{n} \times \vec{S}_1 \cdot \vec{v}_1 - 6 \vec{v}_2 \cdot \vec{v}_2 \hat{n} \times \vec{S}_1 \cdot \vec{v}_1 \right)}{r^4} - \frac{8 G^3 m_1 m_2^2 \vec{S}_1 \times \vec{v}_1 \cdot \vec{a}_1}{r^3} \}$$

$\{\text{DiagSet}[3, 6, 37],$ 
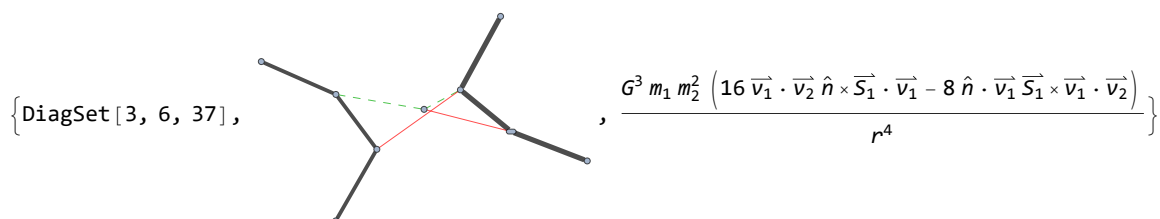
 $,$ 
 $\frac{G^3 m_1 m_2^2 \left( 16 \vec{v}_1 \cdot \vec{v}_2 \hat{n} \times \vec{S}_1 \cdot \vec{v}_1 - 8 \hat{n} \cdot \vec{v}_1 \vec{S}_1 \times \vec{v}_1 \cdot \vec{v}_2 \right)}{r^4} \}$

$\{\text{DiagSet}[3, 6, 38],$ 
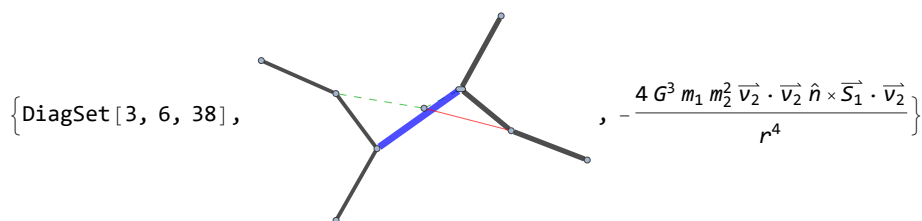
 $,$ 
 $-\frac{4 G^3 m_1 m_2^2 \vec{v}_2 \cdot \vec{v}_2 \hat{n} \times \vec{S}_1 \cdot \vec{v}_2}{r^4} \}$

{DiagSet[3, 6, 39],

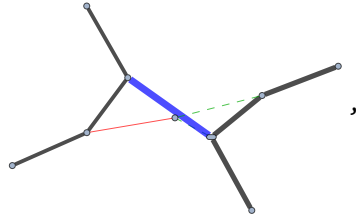

,

$$\frac{G^3 m_1 m_2^2 \left( -4 \hat{n} \cdot \vec{v}_2 \vec{S}_1 \times \vec{v}_1 \cdot \vec{v}_2 - 4 \vec{v}_1 \cdot \vec{v}_2 \hat{n} \times \vec{S}_1 \cdot \vec{v}_2 + 8 \vec{v}_2 \cdot \vec{v}_2 \hat{n} \times \vec{S}_1 \cdot \vec{v}_1 \right)}{r^4} \}$$

{DiagSet[3, 6, 40],

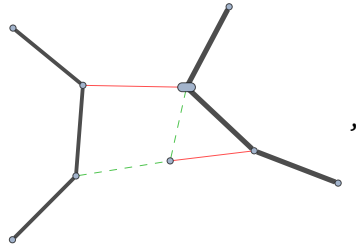

,

$$\frac{G^3 m_1 m_2^2 \left( 16 \hat{n} \cdot \vec{v}_2 \vec{S}_1 \times \vec{v}_1 \cdot \vec{v}_2 + 12 \vec{v}_1 \cdot \vec{v}_1 \hat{n} \times \vec{S}_1 \cdot \vec{v}_2 + 16 \vec{v}_2 \cdot \vec{v}_2 \hat{n} \times \vec{S}_1 \cdot \vec{v}_2 \right)}{r^4} \}$$

{DiagSet[3, 6, 41],

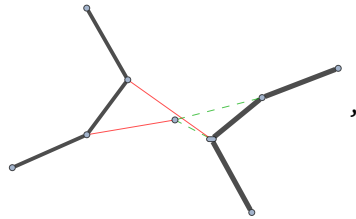

$$, \frac{G^3 m_1 m_2^2 \left( -4 \vec{v}_1 \cdot \vec{v}_1 \hat{n} \times \vec{S}_1 \cdot \vec{v}_1 - 24 \vec{v}_2 \cdot \vec{v}_2 \hat{n} \times \vec{S}_1 \cdot \vec{v}_1 \right)}{r^4} \}$$

{DiagSet[3, 6, 42],

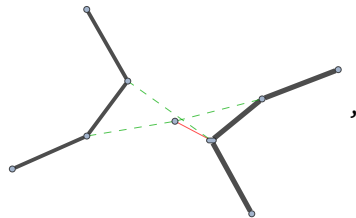

$$, - \frac{64 G^3 m_1 m_2^2 \vec{v}_1 \cdot \vec{v}_2 \hat{n} \times \vec{S}_1 \cdot \vec{v}_2}{r^4} \}$$

{DiagSet[3, 6, 43],

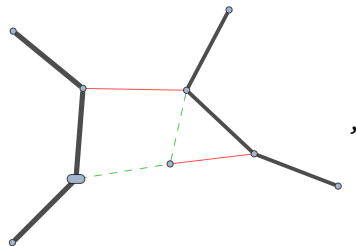

,

$$\frac{G^3 m_1 m_2^2 \left( 8 \vec{a}_1 \times \vec{S}_1 \cdot \vec{v}_2 - 8 \vec{S}_1 \times \vec{v}_1 \cdot \vec{v}_2 \right)}{r^3} + \frac{G^3 m_1 m_2^2 \left( 4 \hat{n} \cdot \vec{v}_1 \vec{S}_1 \times \vec{v}_1 \cdot \vec{v}_2 + 12 \vec{v}_1 \cdot \vec{v}_1 \hat{n} \times \vec{S}_1 \cdot \vec{v}_2 + 12 \vec{v}_1 \cdot \vec{v}_2 \hat{n} \times \vec{S}_1 \cdot \vec{v}_1 \right)}{r^4} \}$$

|                                                                                                                                                                                                                                                                                                                                                                     |                                                                                     |                                                                                                                                                                                        |
|---------------------------------------------------------------------------------------------------------------------------------------------------------------------------------------------------------------------------------------------------------------------------------------------------------------------------------------------------------------------|-------------------------------------------------------------------------------------|----------------------------------------------------------------------------------------------------------------------------------------------------------------------------------------|
| $\{\text{DiagSet}[3, 6, 44],$                                                                                                                                                                                                                                                                                                                                       | 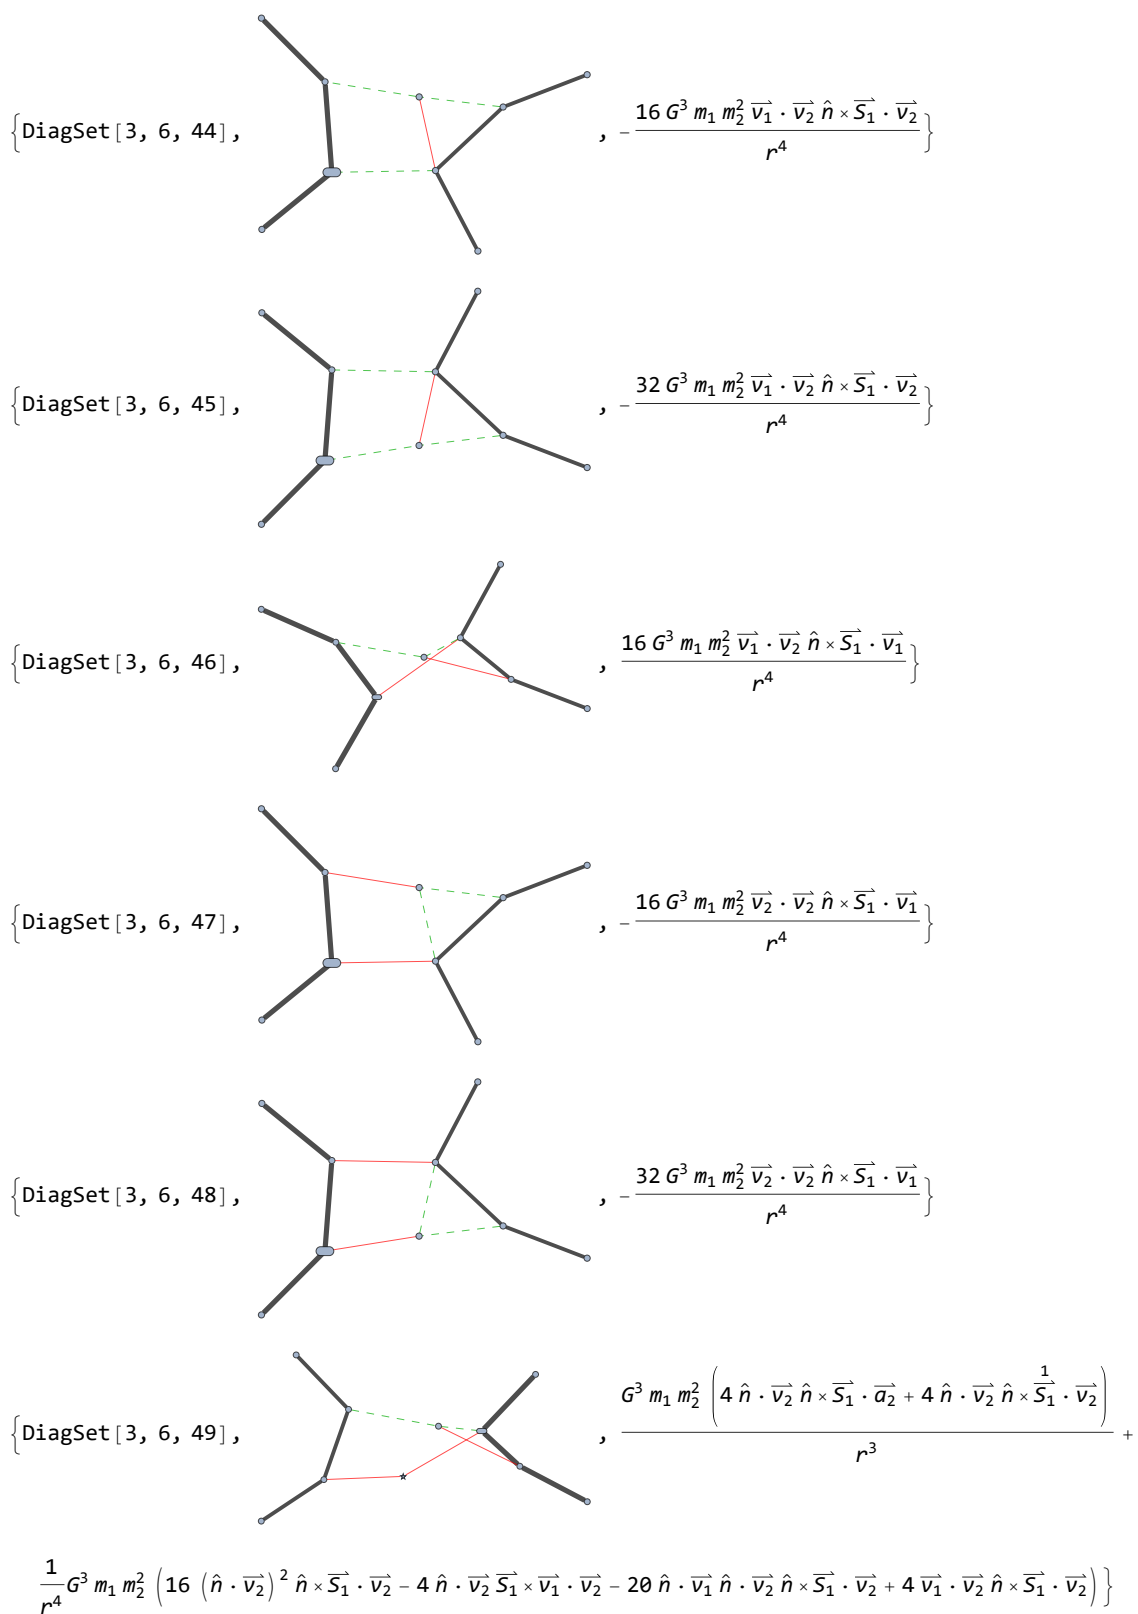   | $, -\frac{16 G^3 m_1 m_2^2 \vec{v}_1 \cdot \vec{v}_2 \hat{n} \times \vec{S}_1 \cdot \vec{v}_2}{r^4} \}$                                                                                |
| $\{\text{DiagSet}[3, 6, 45],$                                                                                                                                                                                                                                                                                                                                       | 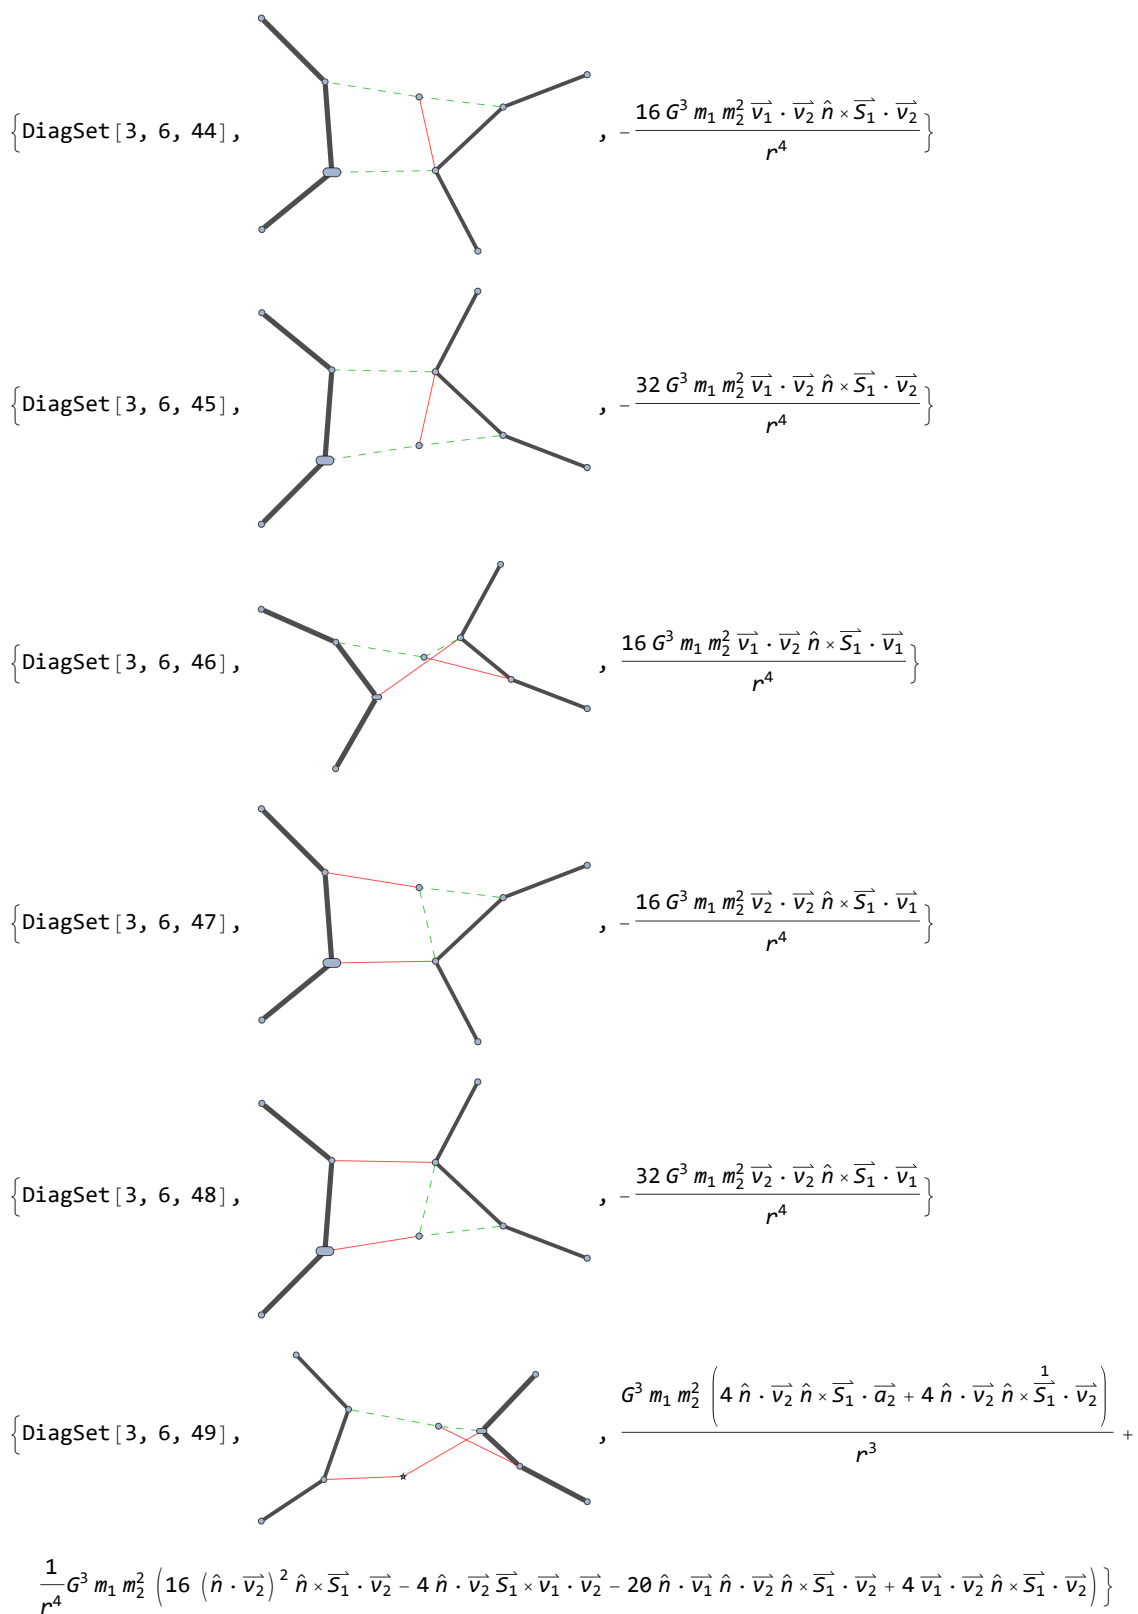   | $, -\frac{32 G^3 m_1 m_2^2 \vec{v}_1 \cdot \vec{v}_2 \hat{n} \times \vec{S}_1 \cdot \vec{v}_2}{r^4} \}$                                                                                |
| $\{\text{DiagSet}[3, 6, 46],$                                                                                                                                                                                                                                                                                                                                       | 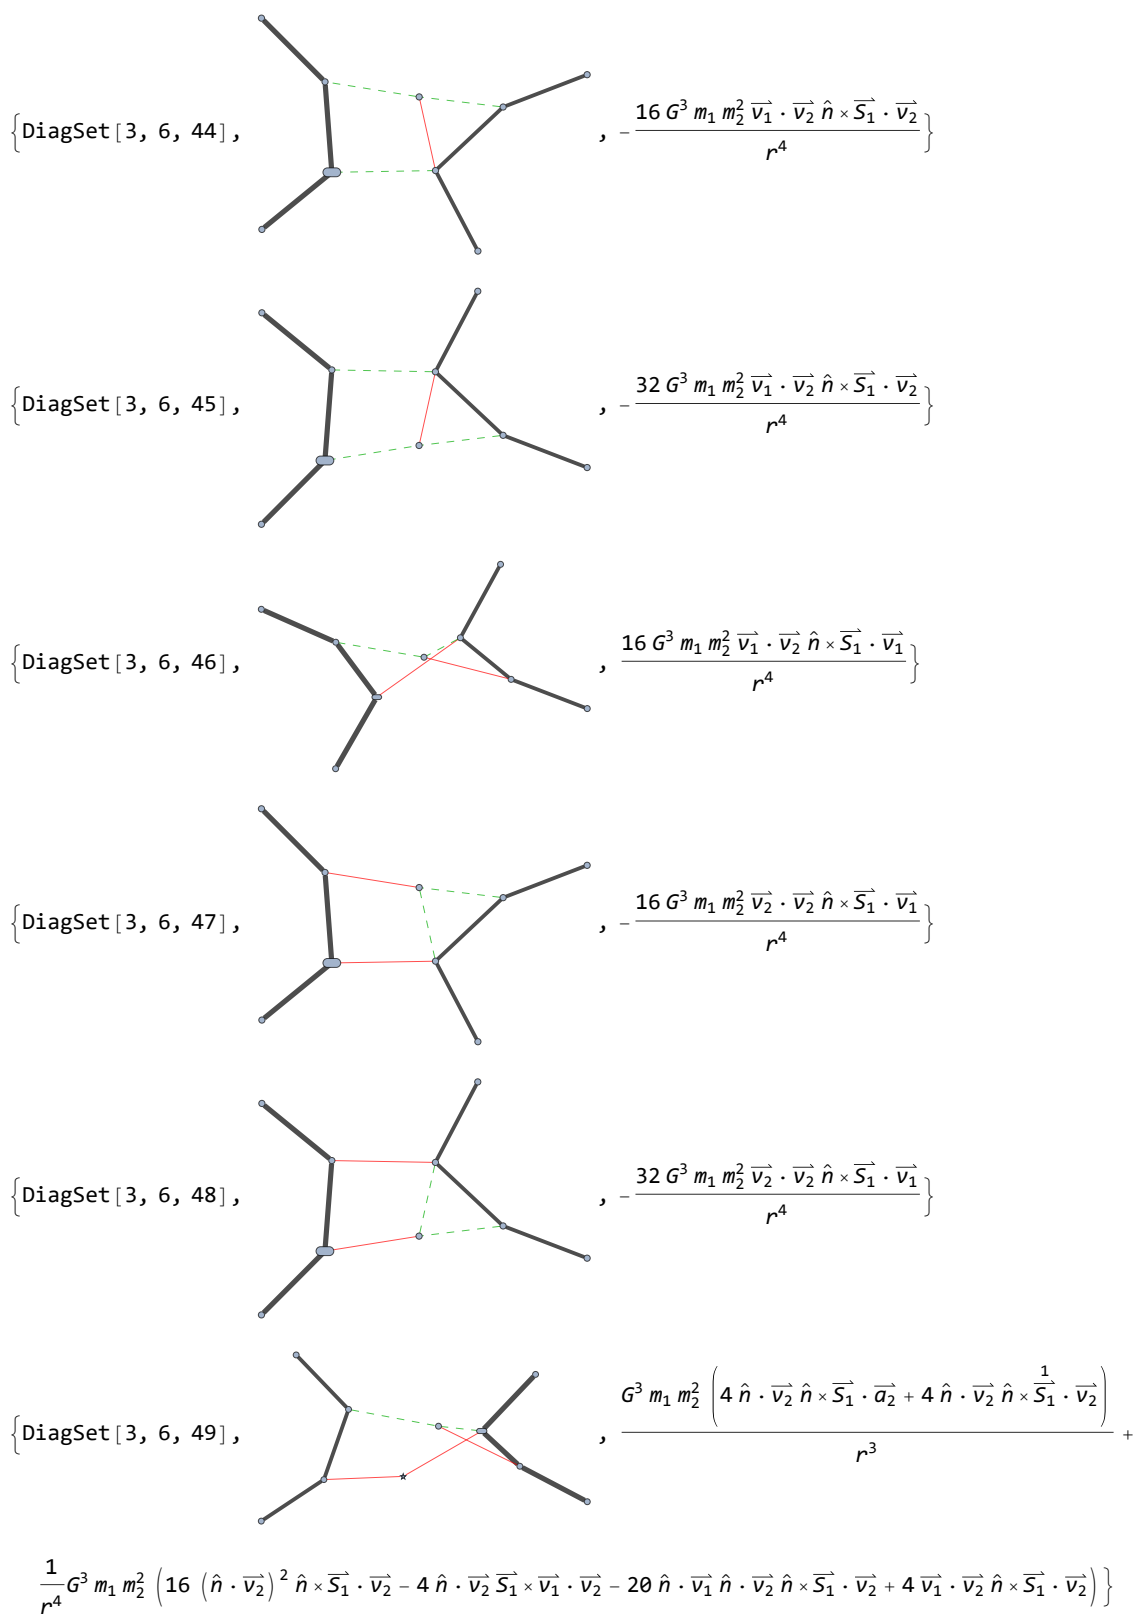  | $, \frac{16 G^3 m_1 m_2^2 \vec{v}_1 \cdot \vec{v}_2 \hat{n} \times \vec{S}_1 \cdot \vec{v}_1}{r^4} \}$                                                                                 |
| $\{\text{DiagSet}[3, 6, 47],$                                                                                                                                                                                                                                                                                                                                       | 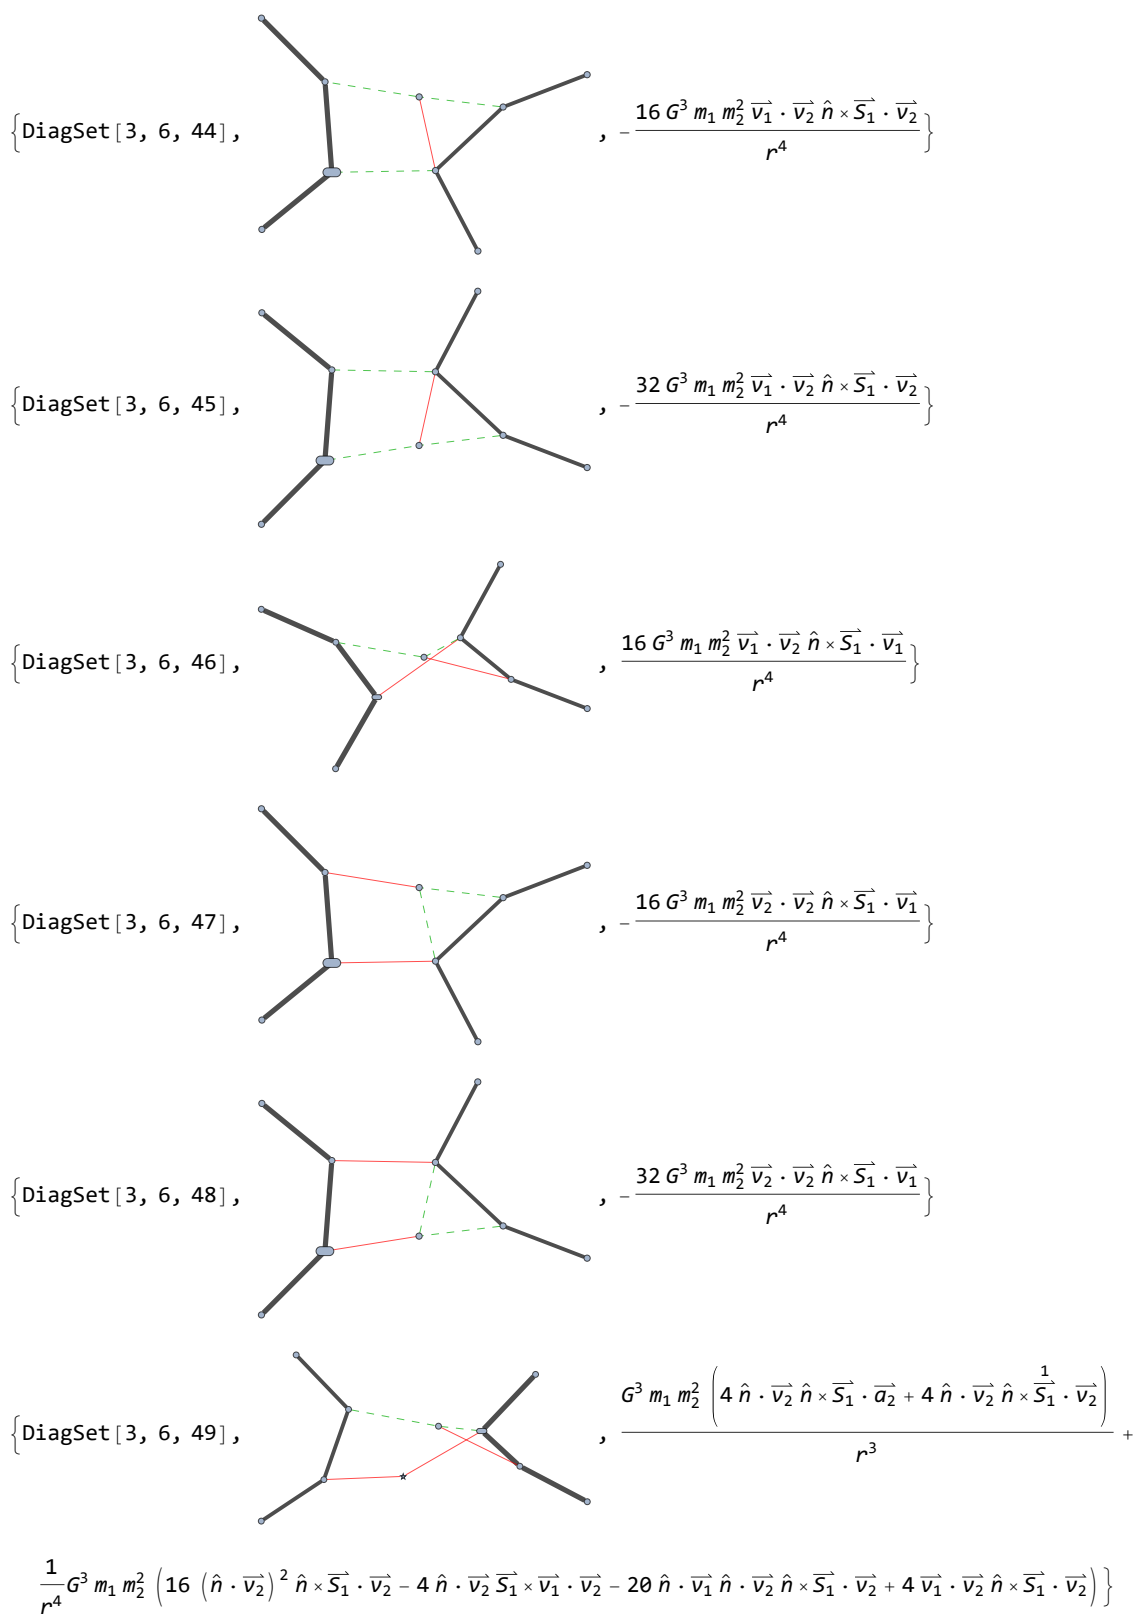 | $, -\frac{16 G^3 m_1 m_2^2 \vec{v}_2 \cdot \vec{v}_2 \hat{n} \times \vec{S}_1 \cdot \vec{v}_1}{r^4} \}$                                                                                |
| $\{\text{DiagSet}[3, 6, 48],$                                                                                                                                                                                                                                                                                                                                       | 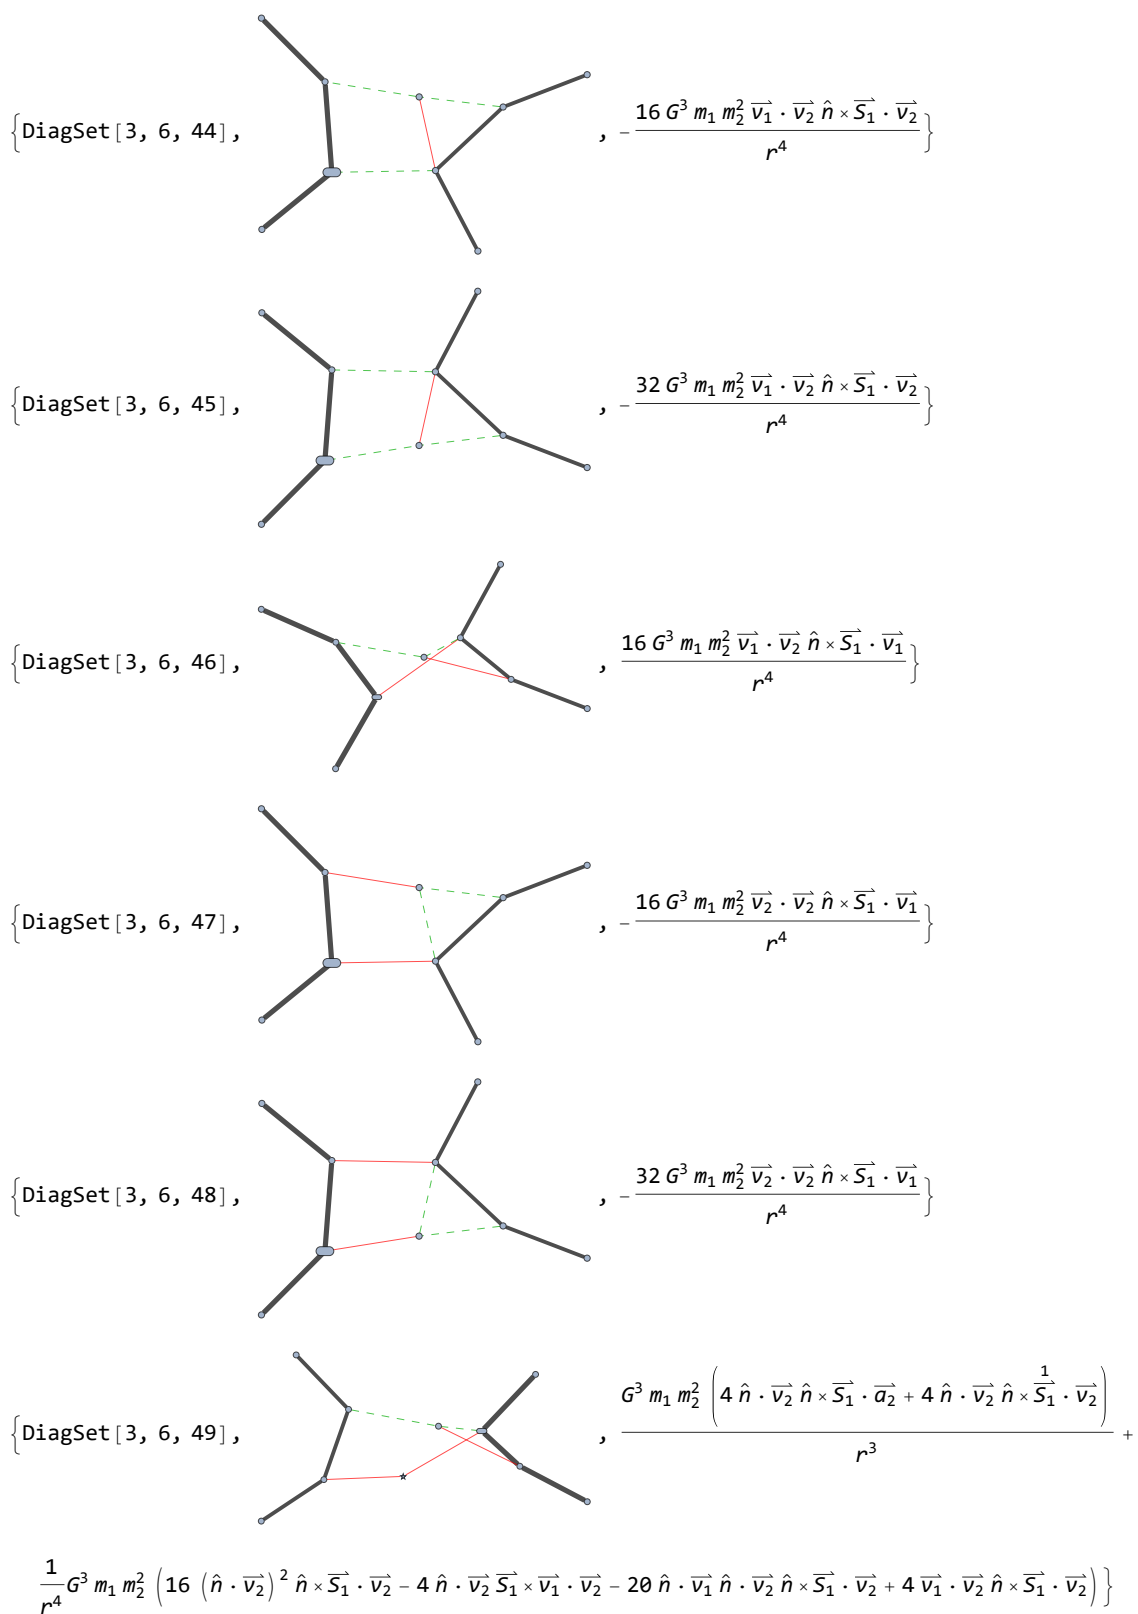 | $, -\frac{32 G^3 m_1 m_2^2 \vec{v}_2 \cdot \vec{v}_2 \hat{n} \times \vec{S}_1 \cdot \vec{v}_1}{r^4} \}$                                                                                |
| $\{\text{DiagSet}[3, 6, 49],$                                                                                                                                                                                                                                                                                                                                       | 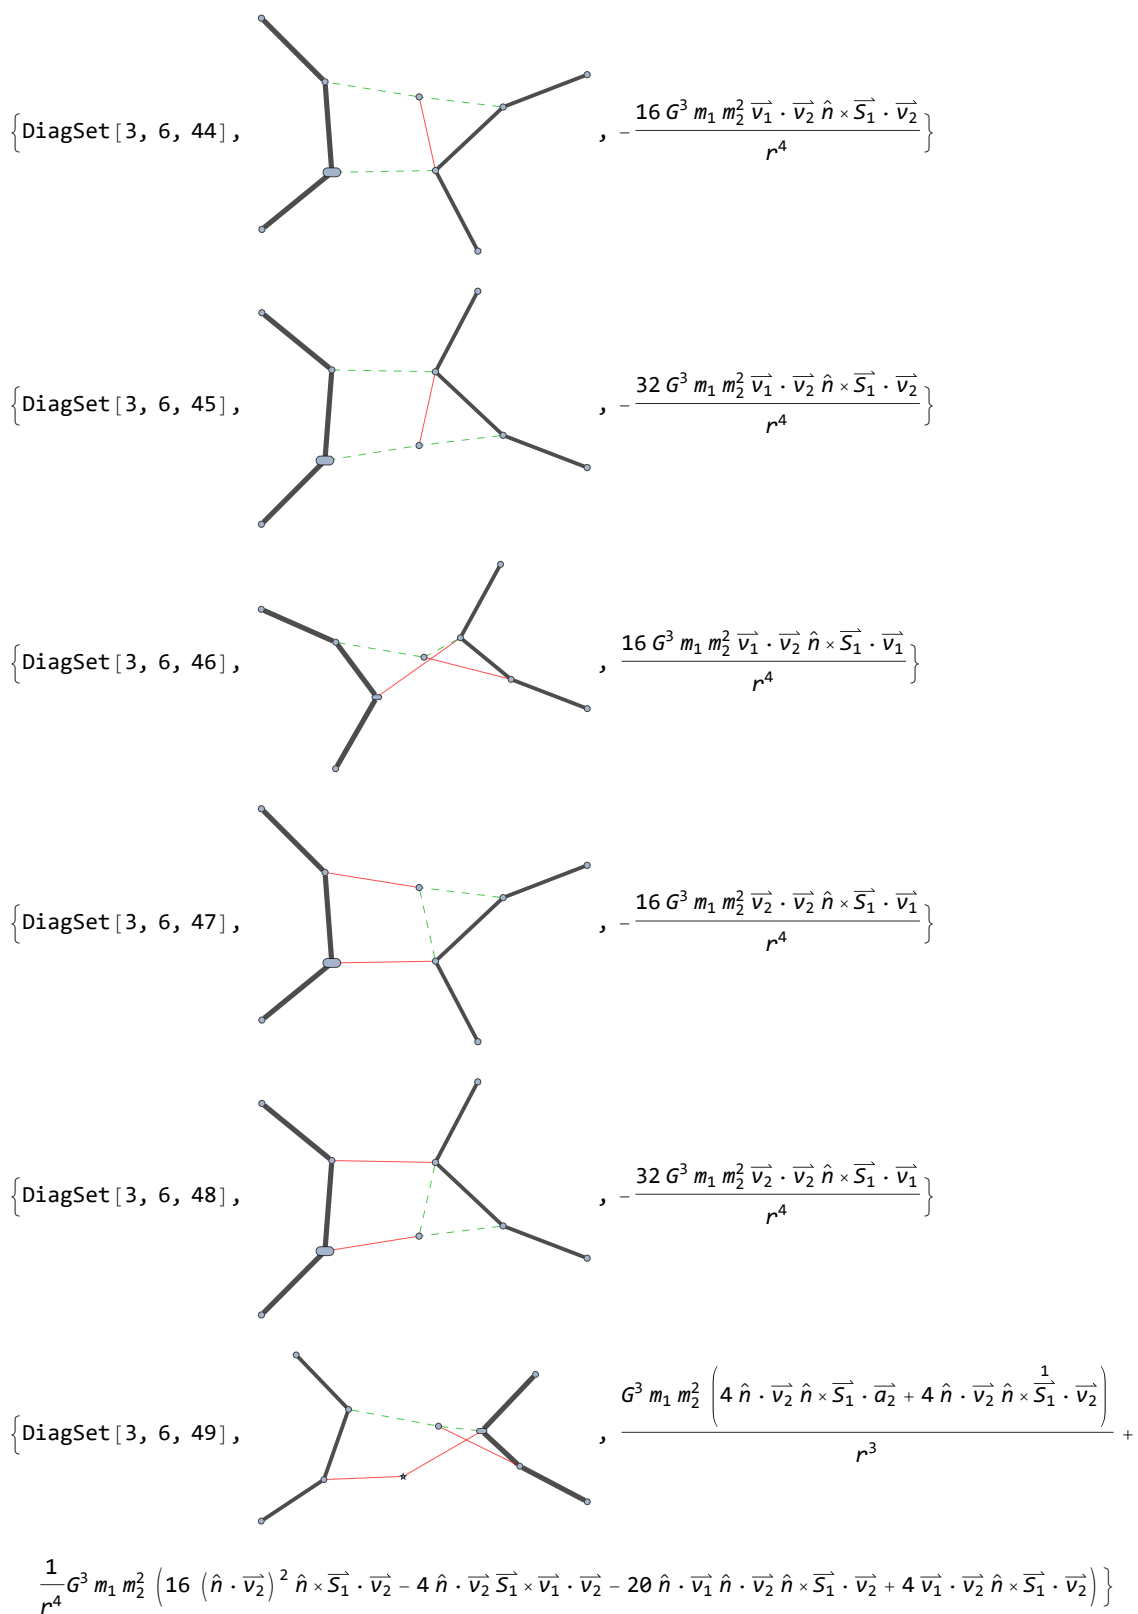 | $, \frac{G^3 m_1 m_2^2 \left( 4 \hat{n} \cdot \vec{v}_2 \hat{n} \times \vec{S}_1 \cdot \vec{a}_2 + 4 \hat{n} \cdot \vec{v}_2 \hat{n} \times \vec{S}_1 \cdot \vec{v}_2 \right)}{r^3} +$ |
| $\frac{1}{r^4} G^3 m_1 m_2^2 \left( 16 (\hat{n} \cdot \vec{v}_2)^2 \hat{n} \times \vec{S}_1 \cdot \vec{v}_2 - 4 \hat{n} \cdot \vec{v}_2 \vec{S}_1 \times \vec{v}_1 \cdot \vec{v}_2 - 20 \hat{n} \cdot \vec{v}_1 \hat{n} \cdot \vec{v}_2 \hat{n} \times \vec{S}_1 \cdot \vec{v}_2 + 4 \vec{v}_1 \cdot \vec{v}_2 \hat{n} \times \vec{S}_1 \cdot \vec{v}_2 \right) \}$ |                                                                                     |                                                                                                                                                                                        |

$\{\text{DiagSet}[3, 6, 50],$  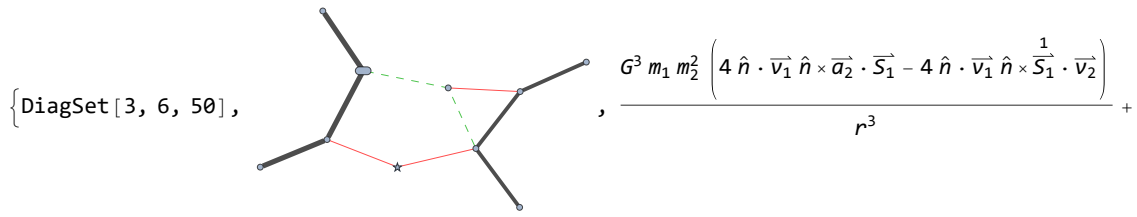 ,  $\frac{G^3 m_1 m_2^2 \left( 4 \hat{n} \cdot \vec{v}_1 \hat{n} \times \vec{a}_2 \cdot \vec{S}_1 - 4 \hat{n} \cdot \vec{v}_1 \hat{n} \times \vec{S}_1 \cdot \vec{v}_2 \right)}{r^3} +$

$\frac{1}{r^4} G^3 m_1 m_2^2 \left( 16 (\hat{n} \cdot \vec{v}_1)^2 \hat{n} \times \vec{S}_1 \cdot \vec{v}_2 + 4 \hat{n} \cdot \vec{v}_1 \vec{S}_1 \times \vec{v}_1 \cdot \vec{v}_2 - 20 \hat{n} \cdot \vec{v}_2 \hat{n} \cdot \vec{v}_1 \hat{n} \times \vec{S}_1 \cdot \vec{v}_2 + 4 \vec{v}_1 \cdot \vec{v}_2 \hat{n} \times \vec{S}_1 \cdot \vec{v}_2 \right) \}$

$\{\text{DiagSet}[3, 6, 51],$  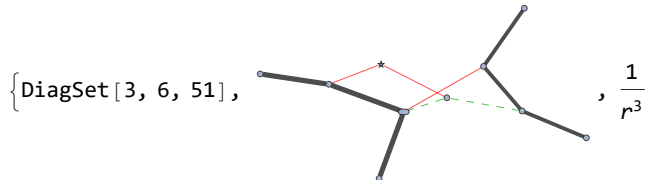 ,  $\frac{1}{r^3}$

$G^3 m_1 m_2^2 \left( 12 \hat{n} \cdot \vec{a}_2 \hat{n} \times \vec{S}_1 \cdot \vec{v}_1 - 8 \hat{n} \cdot \vec{v}_1 \hat{n} \times \vec{S}_1 \cdot \vec{a}_2 - 4 \vec{S}_1 \times \vec{v}_1 \cdot \vec{a}_2 - 8 \hat{n} \cdot \vec{v}_1 \hat{n} \times \vec{S}_1 \cdot \vec{v}_2 + 12 \hat{n} \cdot \vec{v}_2 \hat{n} \times \vec{S}_1 \cdot \vec{v}_1 - 4 \vec{S}_1 \times \vec{v}_1 \cdot \vec{v}_2 \right) +$   
 $\frac{1}{r^4} G^3 m_1 m_2^2 \left( 32 (\hat{n} \cdot \vec{v}_1)^2 \hat{n} \times \vec{S}_1 \cdot \vec{v}_2 + 20 \hat{n} \cdot \vec{v}_1 \vec{S}_1 \times \vec{v}_1 \cdot \vec{v}_2 - 44 \hat{n} \cdot \vec{v}_2 \hat{n} \cdot \vec{v}_1 \hat{n} \times \vec{S}_1 \cdot \vec{v}_1 - 40 \hat{n} \cdot \vec{v}_2 \hat{n} \cdot \vec{v}_1 \hat{n} \times \vec{S}_1 \cdot \vec{v}_2 + \right.$   
 $\left. 60 (\hat{n} \cdot \vec{v}_2)^2 \hat{n} \times \vec{S}_1 \cdot \vec{v}_1 - 24 \hat{n} \cdot \vec{v}_2 \vec{S}_1 \times \vec{v}_1 \cdot \vec{v}_2 + 4 \vec{v}_1 \cdot \vec{v}_2 \hat{n} \times \vec{S}_1 \cdot \vec{v}_1 + 8 \vec{v}_1 \cdot \vec{v}_2 \hat{n} \times \vec{S}_1 \cdot \vec{v}_2 - 12 \vec{v}_2 \cdot \vec{v}_2 \hat{n} \times \vec{S}_1 \cdot \vec{v}_1 \right) \}$

$\{\text{DiagSet}[3, 6, 52],$  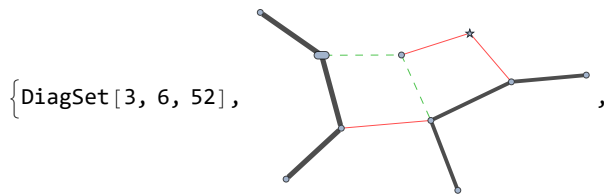 ,

$\frac{G^3 m_1 m_2^2 \left( 4 \hat{n} \cdot \vec{a}_2 \hat{n} \times \vec{S}_1 \cdot \vec{v}_2 - 2 \vec{a}_2 \times \vec{S}_1 \cdot \vec{v}_2 + 4 \hat{n} \cdot \vec{v}_2 \hat{n} \times \vec{S}_1 \cdot \vec{v}_2 \right)}{r^3} + \frac{1}{r^4}$

$G^3 m_1 m_2^2 \left( 16 (\hat{n} \cdot \vec{v}_2)^2 \hat{n} \times \vec{S}_1 \cdot \vec{v}_2 - 4 \hat{n} \cdot \vec{v}_2 \vec{S}_1 \times \vec{v}_1 \cdot \vec{v}_2 - 20 \hat{n} \cdot \vec{v}_1 \hat{n} \cdot \vec{v}_2 \hat{n} \times \vec{S}_1 \cdot \vec{v}_2 + 4 \vec{v}_1 \cdot \vec{v}_2 \hat{n} \times \vec{S}_1 \cdot \vec{v}_2 \right) \}$

$\{\text{DiagSet}[3, 6, 53],$  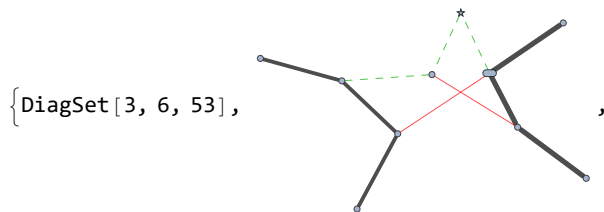 ,

$\frac{1}{r^3} G^3 m_1 m_2^2 \left( -4 \hat{n} \cdot \vec{a}_2 \hat{n} \times \vec{S}_1 \cdot \vec{v}_1 - 48 \hat{n} \cdot \vec{v}_1 \hat{n} \times \vec{S}_1 \cdot \vec{a}_2 + 24 \hat{n} \cdot \vec{v}_2 \hat{n} \times \vec{S}_1 \cdot \vec{a}_2 - \right.$   
 $\left. 12 \vec{S}_1 \times \vec{v}_1 \cdot \vec{a}_2 - 24 \hat{n} \cdot \vec{v}_1 \hat{n} \times \vec{S}_1 \cdot \vec{v}_2 + 4 \hat{n} \cdot \vec{v}_2 \hat{n} \times \vec{S}_1 \cdot \vec{v}_1 + 48 \hat{n} \cdot \vec{v}_2 \hat{n} \times \vec{S}_1 \cdot \vec{v}_2 - 12 \vec{S}_1 \times \vec{v}_1 \cdot \vec{v}_2 \right) +$   
 $\frac{24 G^3 m_1 m_2^2 \hat{n} \times \vec{S}_1 \cdot \vec{a}_2}{r^2} + \frac{1}{r^4} G^3 m_1 m_2^2 \left( 48 (\hat{n} \cdot \vec{v}_1)^2 \hat{n} \times \vec{S}_1 \cdot \vec{v}_2 + 28 \hat{n} \cdot \vec{v}_1 \vec{S}_1 \times \vec{v}_1 \cdot \vec{v}_2 - 4 \hat{n} \cdot \vec{v}_2 \hat{n} \cdot \vec{v}_1 \hat{n} \times \vec{S}_1 \cdot \vec{v}_1 - \right.$   
 $\left. 168 \hat{n} \cdot \vec{v}_2 \hat{n} \cdot \vec{v}_1 \hat{n} \times \vec{S}_1 \cdot \vec{v}_2 - 12 (\hat{n} \cdot \vec{v}_2)^2 \hat{n} \times \vec{S}_1 \cdot \vec{v}_1 + 48 (\hat{n} \cdot \vec{v}_2)^2 \hat{n} \times \vec{S}_1 \cdot \vec{v}_2 - 32 \hat{n} \cdot \vec{v}_2 \vec{S}_1 \times \vec{v}_1 \cdot \vec{v}_2 - \right.$   
 $\left. 8 \vec{v}_1 \cdot \vec{v}_1 \hat{n} \times \vec{S}_1 \cdot \vec{v}_2 - 4 \vec{v}_1 \cdot \vec{v}_2 \hat{n} \times \vec{S}_1 \cdot \vec{v}_1 + 24 \vec{v}_1 \cdot \vec{v}_2 \hat{n} \times \vec{S}_1 \cdot \vec{v}_2 + 4 \vec{v}_2 \cdot \vec{v}_2 \hat{n} \times \vec{S}_1 \cdot \vec{v}_1 \right) \}$

{DiagSet[3, 6, 54],

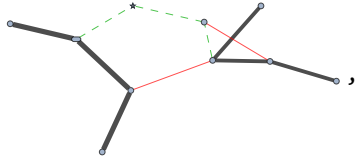

$$\frac{1}{r^3} G^3 m_1 m_2^2 \left( 8 \hat{n} \cdot \vec{v}_1 \hat{n} \times \vec{a}_2 \cdot \vec{S}_1 - 4 \vec{a}_2 \times \vec{S}_1 \cdot \vec{v}_1 - 4 \hat{n} \cdot \vec{v}_1 \hat{n} \times \vec{S}_1 \cdot \vec{v}_2 + 12 \hat{n} \cdot \vec{v}_2 \hat{n} \times \vec{S}_1 \cdot \vec{v}_2 \right) - \frac{4 G^3 m_1 m_2^2 \hat{n} \times \vec{a}_2 \cdot \vec{S}_1}{r^2} + \frac{1}{r^4} G^3 m_1 m_2^2 \left( 8 (\hat{n} \cdot \vec{v}_1)^2 \hat{n} \times \vec{S}_1 \cdot \vec{v}_2 + 4 \hat{n} \cdot \vec{v}_1 \vec{S}_1 \times \vec{v}_1 \cdot \vec{v}_2 - 40 \hat{n} \cdot \vec{v}_2 \hat{n} \cdot \vec{v}_1 \hat{n} \times \vec{S}_1 \cdot \vec{v}_2 - 12 \hat{n} \cdot \vec{v}_2 \vec{S}_1 \times \vec{v}_1 \cdot \vec{v}_2 + 8 \vec{v}_1 \cdot \vec{v}_2 \hat{n} \times \vec{S}_1 \cdot \vec{v}_2 \right) \}$$

{DiagSet[3, 6, 55],

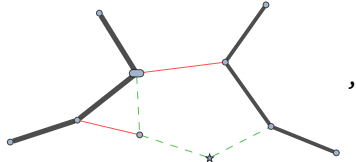

$$\frac{1}{r^3} G^3 m_1 m_2^2 \left( -12 \hat{n} \cdot \vec{v}_1 \hat{n} \times \vec{S}_1 \cdot \vec{a}_2 + 4 \hat{n} \cdot \vec{v}_2 \hat{n} \times \vec{S}_1 \cdot \vec{a}_2 - 4 \vec{S}_1 \times \vec{v}_1 \cdot \vec{a}_2 + 8 \hat{n} \cdot \vec{v}_2 \hat{n} \times \vec{S}_1 \cdot \vec{v}_2 \right) + \frac{4 G^3 m_1 m_2^2 \hat{n} \times \vec{S}_1 \cdot \vec{a}_2}{r^2} + \frac{1}{r^4} G^3 m_1 m_2^2 \left( 8 (\hat{n} \cdot \vec{v}_2)^2 \hat{n} \times \vec{S}_1 \cdot \vec{v}_2 - 8 \hat{n} \cdot \vec{v}_2 \vec{S}_1 \times \vec{v}_1 \cdot \vec{v}_2 - 40 \hat{n} \cdot \vec{v}_1 \hat{n} \cdot \vec{v}_2 \hat{n} \times \vec{S}_1 \cdot \vec{v}_2 + 8 \vec{v}_1 \cdot \vec{v}_2 \hat{n} \times \vec{S}_1 \cdot \vec{v}_2 \right) \}$$

{DiagSet[3, 6, 56],

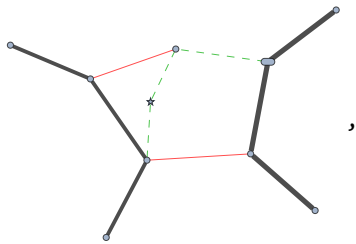

$$\frac{1}{r^3} G^3 m_1 m_2^2 \left( 4 \hat{n} \cdot \vec{a}_2 \hat{n} \times \vec{S}_1 \cdot \vec{v}_2 + 8 \hat{n} \cdot \vec{v}_1 \hat{n} \times \vec{a}_2 \cdot \vec{S}_1 - 4 \vec{a}_2 \times \vec{S}_1 \cdot \vec{v}_1 - 2 \vec{a}_2 \times \vec{S}_1 \cdot \vec{v}_2 - 4 \hat{n} \cdot \vec{v}_1 \hat{n} \times \vec{S}_1 \cdot \vec{v}_2 + 8 \hat{n} \cdot \vec{v}_2 \hat{n} \times \vec{S}_1 \cdot \vec{v}_2 \right) - \frac{4 G^3 m_1 m_2^2 \hat{n} \times \vec{a}_2 \cdot \vec{S}_1}{r^2} + \frac{1}{r^4} G^3 m_1 m_2^2 \left( 8 (\hat{n} \cdot \vec{v}_1)^2 \hat{n} \times \vec{S}_1 \cdot \vec{v}_2 + 4 \hat{n} \cdot \vec{v}_1 \vec{S}_1 \times \vec{v}_1 \cdot \vec{v}_2 - 28 \hat{n} \cdot \vec{v}_2 \hat{n} \cdot \vec{v}_1 \hat{n} \times \vec{S}_1 \cdot \vec{v}_2 + 8 (\hat{n} \cdot \vec{v}_2)^2 \hat{n} \times \vec{S}_1 \cdot \vec{v}_2 - 8 \hat{n} \cdot \vec{v}_2 \vec{S}_1 \times \vec{v}_1 \cdot \vec{v}_2 + 4 \vec{v}_1 \cdot \vec{v}_2 \hat{n} \times \vec{S}_1 \cdot \vec{v}_2 \right) \}$$

{DiagSet[3, 6, 57],

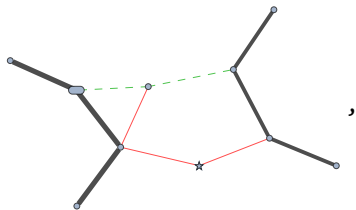

$$, \frac{G^3 m_1 m_2^2 \left( \hat{n} \cdot \vec{v}_2 \hat{n} \times \vec{S}_1 \cdot \vec{a}_2 + \hat{n} \cdot \vec{v}_2 \hat{n} \times \vec{S}_1 \cdot \vec{v}_2 \right)}{r^3} +$$

$$\frac{1}{r^4} G^3 m_1 m_2^2 \left( 4 (\hat{n} \cdot \vec{v}_2)^2 \hat{n} \times \vec{S}_1 \cdot \vec{v}_2 - \hat{n} \cdot \vec{v}_2 \vec{S}_1 \times \vec{v}_1 \cdot \vec{v}_2 - 5 \hat{n} \cdot \vec{v}_1 \hat{n} \cdot \vec{v}_2 \hat{n} \times \vec{S}_1 \cdot \vec{v}_2 + \vec{v}_1 \cdot \vec{v}_2 \hat{n} \times \vec{S}_1 \cdot \vec{v}_2 \right) \}$$

{DiagSet[3, 6, 58],

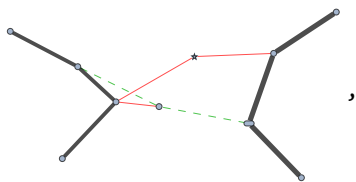

$$, \frac{G^3 m_1 m_2^2 \left( 4 \hat{n} \cdot \vec{v}_1 \hat{n} \times \vec{a}_2 \cdot \vec{S}_1 - 4 \hat{n} \cdot \vec{v}_1 \hat{n} \times \vec{S}_1 \cdot \vec{v}_2 \right)}{r^3} +$$

$$\frac{1}{r^4} G^3 m_1 m_2^2 \left( 16 (\hat{n} \cdot \vec{v}_1)^2 \hat{n} \times \vec{S}_1 \cdot \vec{v}_2 + 4 \hat{n} \cdot \vec{v}_1 \vec{S}_1 \times \vec{v}_1 \cdot \vec{v}_2 - 20 \hat{n} \cdot \vec{v}_2 \hat{n} \cdot \vec{v}_1 \hat{n} \times \vec{S}_1 \cdot \vec{v}_2 + 4 \vec{v}_1 \cdot \vec{v}_2 \hat{n} \times \vec{S}_1 \cdot \vec{v}_2 \right) \}$$



{DiagSet[3, 6, 59],

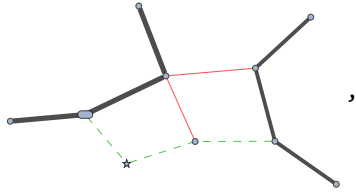

,

$$\frac{1}{r^3} G^3 m_1 m_2^2 \left( -\hat{n} \cdot \vec{a}_2 \hat{n} \times \vec{S}_1 \cdot \vec{v}_1 - 6 \hat{n} \cdot \vec{v}_1 \hat{n} \times \vec{S}_1 \cdot \vec{a}_2 - 3 \vec{S}_1 \times \vec{v}_1 \cdot \vec{a}_2 - 12 \hat{n} \cdot \vec{v}_1 \hat{n} \times \vec{S}_1 \cdot \vec{v}_2 + \right. \\ \left. \hat{n} \cdot \vec{v}_2 \hat{n} \times \vec{S}_1 \cdot \vec{v}_1 + 18 \hat{n} \cdot \vec{v}_2 \hat{n} \times \vec{S}_1 \cdot \vec{v}_2 - 3 \vec{S}_1 \times \vec{v}_1 \cdot \vec{v}_2 \right) + \frac{6 G^3 m_1 m_2^2 \hat{n} \times \vec{S}_1 \cdot \vec{a}_2}{r^2} + \frac{1}{r^4} \\ G^3 m_1 m_2^2 \left( 12 (\hat{n} \cdot \vec{v}_1)^2 \hat{n} \times \vec{S}_1 \cdot \vec{v}_2 + 7 \hat{n} \cdot \vec{v}_1 \vec{S}_1 \times \vec{v}_1 \cdot \vec{v}_2 + \hat{n} \cdot \vec{v}_2 \hat{n} \cdot \vec{v}_1 \hat{n} \times \vec{S}_1 \cdot \vec{v}_1 - 30 \hat{n} \cdot \vec{v}_2 \hat{n} \cdot \vec{v}_1 \hat{n} \times \vec{S}_1 \cdot \vec{v}_2 - 5 (\hat{n} \cdot \vec{v}_2)^2 \right. \\ \left. \hat{n} \times \vec{S}_1 \cdot \vec{v}_1 - 8 \hat{n} \cdot \vec{v}_2 \vec{S}_1 \times \vec{v}_1 \cdot \vec{v}_2 - 2 \vec{v}_1 \cdot \vec{v}_1 \hat{n} \times \vec{S}_1 \cdot \vec{v}_2 - \vec{v}_1 \cdot \vec{v}_2 \hat{n} \times \vec{S}_1 \cdot \vec{v}_1 + 6 \vec{v}_1 \cdot \vec{v}_2 \hat{n} \times \vec{S}_1 \cdot \vec{v}_2 + \vec{v}_2 \cdot \vec{v}_2 \hat{n} \times \vec{S}_1 \cdot \vec{v}_1 \right) \}$$

{DiagSet[3, 6, 60],

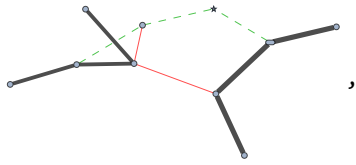

,

$$\frac{1}{r^3} G^3 m_1 m_2^2 \left( 8 \hat{n} \cdot \vec{v}_1 \hat{n} \times \vec{a}_2 \cdot \vec{S}_1 - 4 \vec{a}_2 \times \vec{S}_1 \cdot \vec{v}_1 - 4 \hat{n} \cdot \vec{v}_1 \hat{n} \times \vec{S}_1 \cdot \vec{v}_2 + 12 \hat{n} \cdot \vec{v}_2 \hat{n} \times \vec{S}_1 \cdot \vec{v}_2 \right) - \frac{4 G^3 m_1 m_2^2 \hat{n} \times \vec{a}_2 \cdot \vec{S}_1}{r^2} + \frac{1}{r^4} G^3 m_1 m_2^2 \\ \left( 8 (\hat{n} \cdot \vec{v}_1)^2 \hat{n} \times \vec{S}_1 \cdot \vec{v}_2 + 4 \hat{n} \cdot \vec{v}_1 \vec{S}_1 \times \vec{v}_1 \cdot \vec{v}_2 - 40 \hat{n} \cdot \vec{v}_2 \hat{n} \cdot \vec{v}_1 \hat{n} \times \vec{S}_1 \cdot \vec{v}_2 - 12 \hat{n} \cdot \vec{v}_2 \vec{S}_1 \times \vec{v}_1 \cdot \vec{v}_2 + 8 \vec{v}_1 \cdot \vec{v}_2 \hat{n} \times \vec{S}_1 \cdot \vec{v}_2 \right) \}$$

{DiagSet[3, 6, 61],

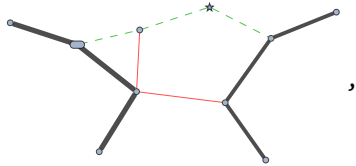

,

$$\frac{1}{r^3} G^3 m_1 m_2^2 \left( -3 \hat{n} \cdot \vec{v}_1 \hat{n} \times \vec{S}_1 \cdot \vec{a}_2 + \hat{n} \cdot \vec{v}_2 \hat{n} \times \vec{S}_1 \cdot \vec{a}_2 - (\vec{S}_1 \times \vec{v}_1 \cdot \vec{a}_2) + 2 \hat{n} \cdot \vec{v}_2 \hat{n} \times \vec{S}_1 \cdot \vec{v}_2 \right) + \frac{G^3 m_1 m_2^2 \hat{n} \times \vec{S}_1 \cdot \vec{a}_2}{r^2} + \\ \frac{1}{r^4} G^3 m_1 m_2^2 \left( 2 (\hat{n} \cdot \vec{v}_2)^2 \hat{n} \times \vec{S}_1 \cdot \vec{v}_2 - 2 \hat{n} \cdot \vec{v}_2 \vec{S}_1 \times \vec{v}_1 \cdot \vec{v}_2 - 10 \hat{n} \cdot \vec{v}_1 \hat{n} \cdot \vec{v}_2 \hat{n} \times \vec{S}_1 \cdot \vec{v}_2 + 2 \vec{v}_1 \cdot \vec{v}_2 \hat{n} \times \vec{S}_1 \cdot \vec{v}_2 \right) \}$$

{DiagSet[3, 6, 62],

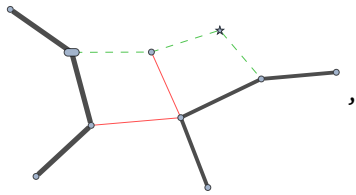

,

$$\frac{1}{r^3} G^3 m_1 m_2^2 \left( 4 \hat{n} \cdot \vec{a}_2 \hat{n} \times \vec{S}_1 \cdot \vec{v}_2 + 12 \hat{n} \cdot \vec{v}_1 \hat{n} \times \vec{a}_2 \cdot \vec{S}_1 - 4 \hat{n} \cdot \vec{v}_2 \hat{n} \times \vec{a}_2 \cdot \vec{S}_1 - 4 \vec{a}_2 \times \vec{S}_1 \cdot \vec{v}_1 - 2 \vec{a}_2 \times \vec{S}_1 \cdot \vec{v}_2 + 4 \hat{n} \cdot \vec{v}_2 \hat{n} \times \vec{S}_1 \cdot \vec{v}_2 \right) - \\ \frac{4 G^3 m_1 m_2^2 \hat{n} \times \vec{a}_2 \cdot \vec{S}_1}{r^2} + \frac{1}{r^4} \\ G^3 m_1 m_2^2 \left( 8 (\hat{n} \cdot \vec{v}_2)^2 \hat{n} \times \vec{S}_1 \cdot \vec{v}_2 - 4 \hat{n} \cdot \vec{v}_2 \vec{S}_1 \times \vec{v}_1 \cdot \vec{v}_2 - 20 \hat{n} \cdot \vec{v}_1 \hat{n} \cdot \vec{v}_2 \hat{n} \times \vec{S}_1 \cdot \vec{v}_2 + 4 \vec{v}_1 \cdot \vec{v}_2 \hat{n} \times \vec{S}_1 \cdot \vec{v}_2 \right) \}$$

$$\left\{ \text{DiagSet}[3, 6, 63], \right.$$
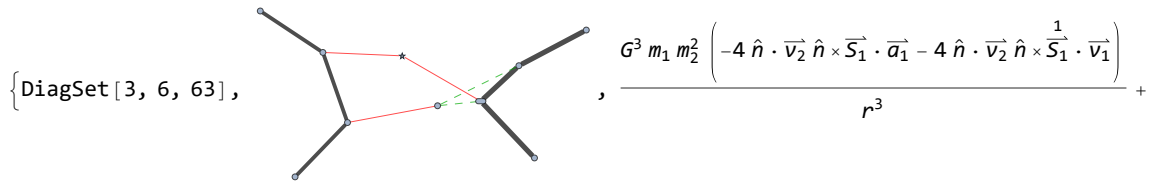

$$, \frac{G^3 m_1 m_2^2 \left( -4 \hat{n} \cdot \vec{v}_2 \hat{n} \times \vec{S}_1 \cdot \vec{a}_1 - 4 \hat{n} \cdot \vec{v}_2 \hat{n} \times \vec{S}_1 \cdot \vec{v}_1 \right)}{r^3} +$$

$$\frac{1}{r^4} G^3 m_1 m_2^2 \left( -16 (\hat{n} \cdot \vec{v}_2)^2 \hat{n} \times \vec{S}_1 \cdot \vec{v}_1 + 4 \hat{n} \cdot \vec{v}_2 \vec{S}_1 \times \vec{v}_1 \cdot \vec{v}_2 + 20 \hat{n} \cdot \vec{v}_1 \hat{n} \cdot \vec{v}_2 \hat{n} \times \vec{S}_1 \cdot \vec{v}_1 - 4 \vec{v}_1 \cdot \vec{v}_2 \hat{n} \times \vec{S}_1 \cdot \vec{v}_1 \right) \}$$

$$\left\{ \text{DiagSet}[3, 6, 64], \right.$$
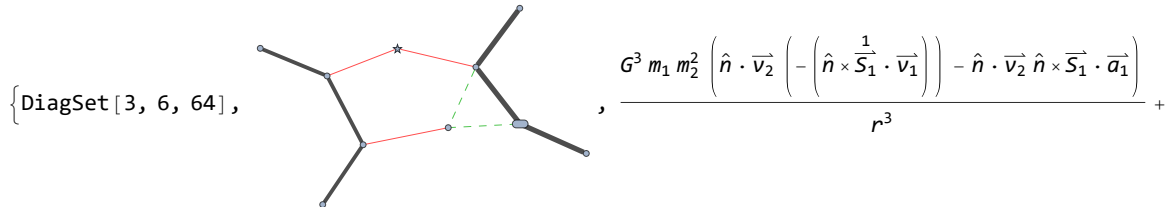

$$, \frac{G^3 m_1 m_2^2 \left( \hat{n} \cdot \vec{v}_2 \left( - \left( \hat{n} \times \vec{S}_1 \cdot \vec{v}_1 \right) \right) - \hat{n} \cdot \vec{v}_2 \hat{n} \times \vec{S}_1 \cdot \vec{a}_1 \right)}{r^3} +$$

$$\frac{1}{r^4} G^3 m_1 m_2^2 \left( -4 (\hat{n} \cdot \vec{v}_2)^2 \hat{n} \times \vec{S}_1 \cdot \vec{v}_1 + \hat{n} \cdot \vec{v}_2 \vec{S}_1 \times \vec{v}_1 \cdot \vec{v}_2 + 5 \hat{n} \cdot \vec{v}_1 \hat{n} \cdot \vec{v}_2 \hat{n} \times \vec{S}_1 \cdot \vec{v}_1 - \vec{v}_1 \cdot \vec{v}_2 \hat{n} \times \vec{S}_1 \cdot \vec{v}_1 \right) \}$$

$$\left\{ \text{DiagSet}[3, 6, 65], \right.$$
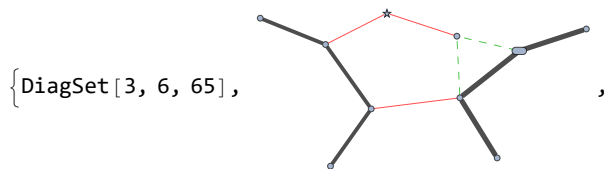

$$,$$

$$\frac{G^3 m_1 m_2^2 \left( -2 \hat{n} \cdot \vec{v}_2 \hat{n} \times \vec{S}_1 \cdot \vec{a}_1 + \vec{S}_1 \times \vec{a}_1 \cdot \vec{v}_2 - 2 \hat{n} \cdot \vec{v}_2 \hat{n} \times \vec{S}_1 \cdot \vec{v}_1 + \vec{S}_1 \times \vec{v}_1 \cdot \vec{v}_2 \right)}{r^3} + \frac{1}{r^4}$$

$$G^3 m_1 m_2^2 \left( -2 (\hat{n} \cdot \vec{v}_2)^2 \hat{n} \times \vec{S}_1 \cdot \vec{v}_1 + \hat{n} \cdot \vec{v}_2 \vec{S}_1 \times \vec{v}_1 \cdot \vec{v}_2 + 10 \hat{n} \cdot \vec{v}_1 \hat{n} \cdot \vec{v}_2 \hat{n} \times \vec{S}_1 \cdot \vec{v}_1 - 3 \hat{n} \cdot \vec{v}_1 \vec{S}_1 \times \vec{v}_1 \cdot \vec{v}_2 - 2 \vec{v}_1 \cdot \vec{v}_2 \hat{n} \times \vec{S}_1 \cdot \vec{v}_1 \right) \}$$

$$\left\{ \text{DiagSet}[3, 6, 66], \right.$$
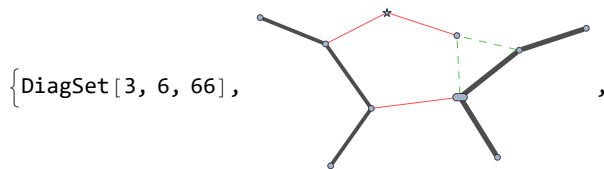

$$,$$

$$\frac{G^3 m_1 m_2^2 \left( -8 \hat{n} \cdot \vec{v}_2 \hat{n} \times \vec{S}_1 \cdot \vec{a}_1 + 4 \vec{S}_1 \times \vec{a}_1 \cdot \vec{v}_2 - 8 \hat{n} \cdot \vec{v}_2 \hat{n} \times \vec{S}_1 \cdot \vec{v}_1 + 4 \vec{S}_1 \times \vec{v}_1 \cdot \vec{v}_2 \right)}{r^3} + \frac{1}{r^4} G^3 m_1 m_2^2$$

$$\left( -8 (\hat{n} \cdot \vec{v}_2)^2 \hat{n} \times \vec{S}_1 \cdot \vec{v}_1 + 4 \hat{n} \cdot \vec{v}_2 \vec{S}_1 \times \vec{v}_1 \cdot \vec{v}_2 + 40 \hat{n} \cdot \vec{v}_1 \hat{n} \cdot \vec{v}_2 \hat{n} \times \vec{S}_1 \cdot \vec{v}_1 - 12 \hat{n} \cdot \vec{v}_1 \vec{S}_1 \times \vec{v}_1 \cdot \vec{v}_2 - 8 \vec{v}_1 \cdot \vec{v}_2 \hat{n} \times \vec{S}_1 \cdot \vec{v}_1 \right) \}$$

$$\left\{ \text{DiagSet}[3, 6, 67], \right.$$
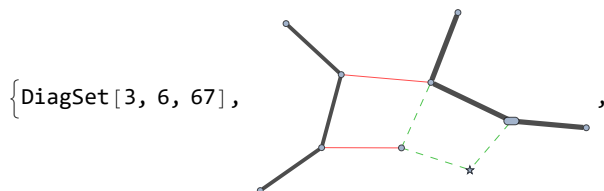

$$,$$

$$\frac{1}{r^3} G^3 m_1 m_2^2 \left( \hat{n} \cdot \vec{a}_1 \hat{n} \times \vec{S}_1 \cdot \vec{v}_1 + \vec{S}_1 \times \vec{v}_1 \cdot \vec{a}_1 + 5 \hat{n} \cdot \vec{v}_1 \hat{n} \times \vec{S}_1 \cdot \vec{v}_1 - 6 \hat{n} \cdot \vec{v}_2 \hat{n} \times \vec{S}_1 \cdot \vec{v}_1 + 2 \vec{S}_1 \times \vec{v}_1 \cdot \vec{v}_2 \right) - \frac{2 G^3 m_1 m_2^2 \hat{n} \times \vec{S}_1 \cdot \vec{a}_1}{r^2} +$$

$$\frac{1}{r^4} G^3 m_1 m_2^2 \left( -3 (\hat{n} \cdot \vec{v}_1)^2 \hat{n} \times \vec{S}_1 \cdot \vec{v}_1 - \hat{n} \cdot \vec{v}_1 \vec{S}_1 \times \vec{v}_1 \cdot \vec{v}_2 + 5 \hat{n} \cdot \vec{v}_2 \hat{n} \cdot \vec{v}_1 \hat{n} \times \vec{S}_1 \cdot \vec{v}_1 + \vec{v}_1 \cdot \vec{v}_1 \hat{n} \times \vec{S}_1 \cdot \vec{v}_1 - \vec{v}_1 \cdot \vec{v}_2 \hat{n} \times \vec{S}_1 \cdot \vec{v}_1 \right) \}$$

{DiagSet[3, 6, 68],

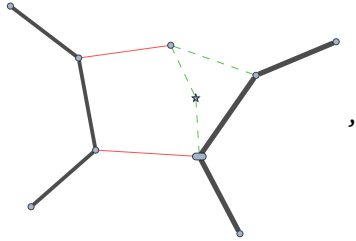

,

$$\begin{aligned} & \frac{1}{r^3} G^3 m_1 m_2^2 \left( 4 \hat{n} \cdot \vec{a}_1 \hat{n} \times \vec{S}_1 \cdot \vec{v}_1 + 8 \hat{n} \cdot \vec{v}_1 \hat{n} \times \vec{S}_1 \cdot \vec{a}_1 - 8 \hat{n} \cdot \vec{v}_2 \hat{n} \times \vec{S}_1 \cdot \vec{a}_1 + \right. \\ & \quad \left. 4 \vec{S}_1 \times \vec{v}_1 \cdot \vec{a}_1 + 12 \hat{n} \cdot \vec{v}_1 \hat{n} \times \vec{S}_1 \cdot \vec{v}_1 - 16 \hat{n} \cdot \vec{v}_2 \hat{n} \times \vec{S}_1 \cdot \vec{v}_1 + 8 \vec{S}_1 \times \vec{v}_1 \cdot \vec{v}_2 \right) - \frac{8 G^3 m_1 m_2^2 \hat{n} \times \vec{S}_1 \cdot \vec{a}_1}{r^2} + \\ & \quad \frac{1}{r^4} G^3 m_1 m_2^2 \left( -20 (\hat{n} \cdot \vec{v}_1)^2 \hat{n} \times \vec{S}_1 \cdot \vec{v}_1 - 12 \hat{n} \cdot \vec{v}_1 \vec{S}_1 \times \vec{v}_1 \cdot \vec{v}_2 + 44 \hat{n} \cdot \vec{v}_2 \hat{n} \cdot \vec{v}_1 \hat{n} \times \vec{S}_1 \cdot \vec{v}_1 - \right. \\ & \quad \left. 16 (\hat{n} \cdot \vec{v}_2)^2 \hat{n} \times \vec{S}_1 \cdot \vec{v}_1 + 8 \hat{n} \cdot \vec{v}_2 \vec{S}_1 \times \vec{v}_1 \cdot \vec{v}_2 + 4 \vec{v}_1 \cdot \vec{v}_1 \hat{n} \times \vec{S}_1 \cdot \vec{v}_1 - 4 \vec{v}_1 \cdot \vec{v}_2 \hat{n} \times \vec{S}_1 \cdot \vec{v}_1 \right) \} \end{aligned}$$

{DiagSet[3, 6, 69],

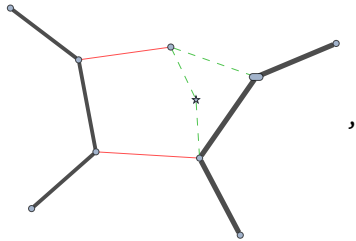

,

$$\begin{aligned} & \frac{1}{r^3} G^3 m_1 m_2^2 \left( 3 \hat{n} \cdot \vec{a}_1 \hat{n} \times \vec{S}_1 \cdot \vec{v}_1 - 6 \hat{n} \cdot \vec{v}_1 \hat{n} \times \vec{S}_1 \cdot \vec{a}_1 + 4 \hat{n} \cdot \vec{v}_2 \hat{n} \times \vec{S}_1 \cdot \vec{a}_1 - \right. \\ & \quad \left. 2 \vec{S}_1 \times \vec{a}_1 \cdot \vec{v}_2 - 3 \vec{S}_1 \times \vec{v}_1 \cdot \vec{a}_1 - 3 \hat{n} \cdot \vec{v}_1 \hat{n} \times \vec{S}_1 \cdot \vec{v}_1 + 2 \hat{n} \cdot \vec{v}_2 \hat{n} \times \vec{S}_1 \cdot \vec{v}_1 \right) + \\ & \quad \frac{2 G^3 m_1 m_2^2 \hat{n} \times \vec{S}_1 \cdot \vec{a}_1}{r^2} + \frac{1}{r^4} G^3 m_1 m_2^2 \left( 5 (\hat{n} \cdot \vec{v}_1)^2 \hat{n} \times \vec{S}_1 \cdot \vec{v}_1 + 3 \hat{n} \cdot \vec{v}_1 \vec{S}_1 \times \vec{v}_1 \cdot \vec{v}_2 - 11 \hat{n} \cdot \vec{v}_2 \hat{n} \cdot \vec{v}_1 \hat{n} \times \vec{S}_1 \cdot \vec{v}_1 + \right. \\ & \quad \left. 4 (\hat{n} \cdot \vec{v}_2)^2 \hat{n} \times \vec{S}_1 \cdot \vec{v}_1 - 2 \hat{n} \cdot \vec{v}_2 \vec{S}_1 \times \vec{v}_1 \cdot \vec{v}_2 - \vec{v}_1 \cdot \vec{v}_1 \hat{n} \times \vec{S}_1 \cdot \vec{v}_1 + \vec{v}_1 \cdot \vec{v}_2 \hat{n} \times \vec{S}_1 \cdot \vec{v}_1 \right) \} \end{aligned}$$

{DiagSet[3, 6, 70],

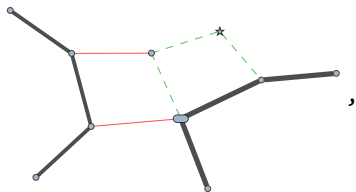

,

$$\begin{aligned} & \frac{1}{r^3} G^3 m_1 m_2^2 \left( 12 \hat{n} \cdot \vec{a}_1 \hat{n} \times \vec{S}_1 \cdot \vec{v}_1 - 32 \hat{n} \cdot \vec{v}_1 \hat{n} \times \vec{S}_1 \cdot \vec{a}_1 + 24 \hat{n} \cdot \vec{v}_2 \hat{n} \times \vec{S}_1 \cdot \vec{a}_1 - \right. \\ & \quad \left. 8 \vec{S}_1 \times \vec{a}_1 \cdot \vec{v}_2 - 12 \vec{S}_1 \times \vec{v}_1 \cdot \vec{a}_1 - 4 \hat{n} \cdot \vec{v}_1 \hat{n} \times \vec{S}_1 \cdot \vec{v}_1 \right) + \frac{8 G^3 m_1 m_2^2 \hat{n} \times \vec{S}_1 \cdot \vec{a}_1}{r^2} + \frac{1}{r^4} G^3 m_1 m_2^2 \\ & \quad \left( 12 (\hat{n} \cdot \vec{v}_1)^2 \hat{n} \times \vec{S}_1 \cdot \vec{v}_1 + 4 \hat{n} \cdot \vec{v}_1 \vec{S}_1 \times \vec{v}_1 \cdot \vec{v}_2 - 20 \hat{n} \cdot \vec{v}_2 \hat{n} \cdot \vec{v}_1 \hat{n} \times \vec{S}_1 \cdot \vec{v}_1 - 4 \vec{v}_1 \cdot \vec{v}_1 \hat{n} \times \vec{S}_1 \cdot \vec{v}_1 + 4 \vec{v}_1 \cdot \vec{v}_2 \hat{n} \times \vec{S}_1 \cdot \vec{v}_1 \right) \} \end{aligned}$$

{DiagSet[3, 6, 71],

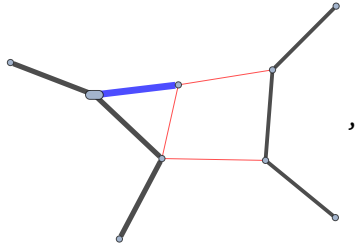

,

$$\frac{1}{r^3} G^3 m_1 m_2^2 \left( -4 \hat{n} \cdot \vec{a}_1 \hat{n} \times \vec{S}_1 \cdot \vec{v}_1 - 8 \hat{n} \cdot \vec{v}_1 \hat{n} \times \vec{S}_1 \cdot \vec{a}_1 - 2 \vec{S}_1 \times \vec{v}_1 \cdot \vec{a}_1 - 6 \hat{n} \cdot \vec{v}_1 \hat{n} \times \vec{S}_1 \cdot \vec{v}_1 \right) + \frac{1}{r^4} G^3 m_1 m_2^2 \left( 4 (\hat{n} \cdot \vec{v}_1)^2 \hat{n} \times \vec{S}_1 \cdot \vec{v}_1 + 3 \hat{n} \cdot \vec{v}_1 \vec{S}_1 \times \vec{v}_1 \cdot \vec{v}_2 - 8 \hat{n} \cdot \vec{v}_2 \hat{n} \cdot \vec{v}_1 \hat{n} \times \vec{S}_1 \cdot \vec{v}_1 + 4 (\hat{n} \cdot \vec{v}_2)^2 \hat{n} \times \vec{S}_1 \cdot \vec{v}_1 - 2 \hat{n} \cdot \vec{v}_2 \vec{S}_1 \times \vec{v}_1 \cdot \vec{v}_2 - \frac{7}{2} \vec{v}_1 \cdot \vec{v}_1 \hat{n} \times \vec{S}_1 \cdot \vec{v}_1 + \vec{v}_1 \cdot \vec{v}_2 \hat{n} \times \vec{S}_1 \cdot \vec{v}_1 + \frac{3}{2} \vec{v}_2 \cdot \vec{v}_2 \hat{n} \times \vec{S}_1 \cdot \vec{v}_1 \right) \Big\}$$

{DiagSet[3, 6, 72],

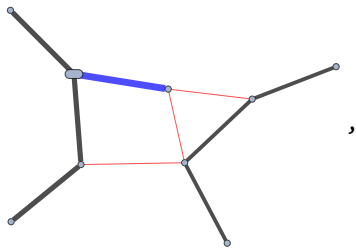

,

$$\frac{G^3 m_1 m_2^2 \left( \hat{n} \cdot \vec{a}_1 \hat{n} \times \vec{S}_1 \cdot \vec{v}_1 - 2 \hat{n} \cdot \vec{v}_1 \hat{n} \times \vec{a}_1 \cdot \vec{S}_1 + \vec{a}_1 \times \vec{S}_1 \cdot \vec{v}_1 + \frac{3}{2} \hat{n} \cdot \vec{v}_1 \hat{n} \times \vec{S}_1 \cdot \vec{v}_1 \right)}{r^3} + \frac{1}{r^4} G^3 m_1 m_2^2 \left( -4 (\hat{n} \cdot \vec{v}_1)^2 \hat{n} \times \vec{S}_1 \cdot \vec{v}_1 + 2 \hat{n} \cdot \vec{v}_1 \vec{S}_1 \times \vec{v}_1 \cdot \vec{v}_2 - 4 \hat{n} \cdot \vec{v}_2 \hat{n} \cdot \vec{v}_1 \hat{n} \times \vec{S}_1 \cdot \vec{v}_1 + 8 (\hat{n} \cdot \vec{v}_2)^2 \hat{n} \times \vec{S}_1 \cdot \vec{v}_1 - 4 \hat{n} \cdot \vec{v}_2 \vec{S}_1 \times \vec{v}_1 \cdot \vec{v}_2 + 3 \vec{v}_1 \cdot \vec{v}_1 \hat{n} \times \vec{S}_1 \cdot \vec{v}_1 - 5 \vec{v}_2 \cdot \vec{v}_2 \hat{n} \times \vec{S}_1 \cdot \vec{v}_1 \right) \Big\}$$

{DiagSet[3, 6, 73],

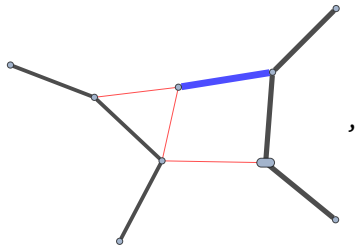

$$\left\{ \frac{G^3 m_1 m_2^2 \left( 2 \vec{v}_1 \cdot \vec{v}_1 \hat{n} \times \vec{S}_1 \cdot \vec{v}_1 - 2 (\hat{n} \cdot \vec{v}_1)^2 \hat{n} \times \vec{S}_1 \cdot \vec{v}_1 \right)}{r^4} \right\}$$

{DiagSet[3, 6, 74],

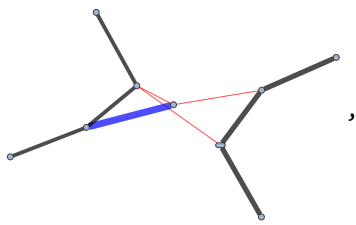

$$\left\{ \frac{G^3 m_1 m_2^2 \left( 8 (\hat{n} \cdot \vec{v}_2)^2 \hat{n} \times \vec{S}_1 \cdot \vec{v}_1 - 4 \vec{v}_2 \cdot \vec{v}_2 \hat{n} \times \vec{S}_1 \cdot \vec{v}_1 \right)}{r^4} \right\}$$

{DiagSet[3, 6, 75],

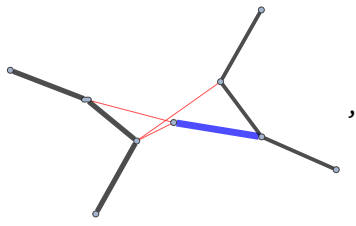

,

$$\frac{G^3 m_1 m_2^2 \left( -4 \left( \hat{n} \cdot \vec{v}_2 \right)^2 \hat{n} \times \vec{S}_1 \cdot \vec{v}_1 + 2 \hat{n} \cdot \vec{v}_2 \vec{S}_1 \times \vec{v}_1 \cdot \vec{v}_2 + 2 \vec{v}_2 \cdot \vec{v}_2 \hat{n} \times \vec{S}_1 \cdot \vec{v}_1 \right)}{r^4} \}$$

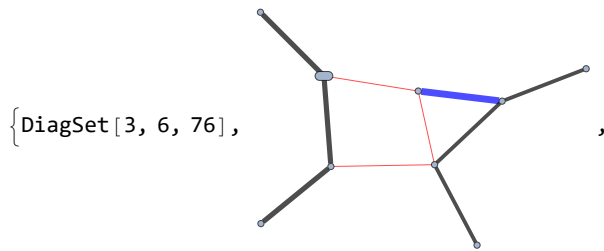

$$\frac{G^3 m_1 m_2^2 \left( 32 \left( \hat{n} \cdot \vec{v}_2 \right)^2 \hat{n} \times \vec{S}_1 \cdot \vec{v}_1 - 16 \hat{n} \cdot \vec{v}_2 \vec{S}_1 \times \vec{v}_1 \cdot \vec{v}_2 - 8 \vec{v}_2 \cdot \vec{v}_2 \hat{n} \times \vec{S}_1 \cdot \vec{v}_1 \right)}{r^4} \}$$

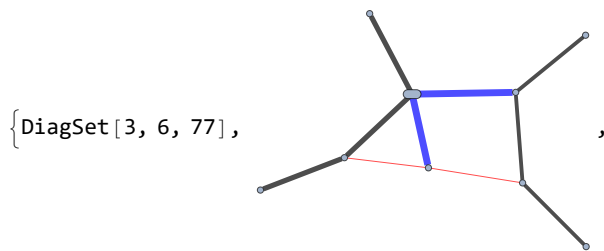

$$\frac{G^3 m_1 m_2^2 \left( 4 \hat{n} \cdot \vec{a}_2 \hat{n} \times \vec{S}_1 \cdot \vec{v}_2 + 4 \hat{n} \cdot \vec{v}_2 \hat{n} \times \vec{S}_1 \cdot \vec{a}_2 \right)}{r^3} + \frac{1}{r^4} G^3 m_1 m_2^2 \left( -12 \left( \hat{n} \cdot \vec{v}_2 \right)^2 \hat{n} \times \vec{S}_1 \cdot \vec{v}_2 + 5 \hat{n} \cdot \vec{v}_2 \vec{S}_1 \times \vec{v}_1 \cdot \vec{v}_2 + \right. \\ \left. 12 \hat{n} \cdot \vec{v}_1 \hat{n} \cdot \vec{v}_2 \hat{n} \times \vec{S}_1 \cdot \vec{v}_2 - 3 \vec{v}_1 \cdot \vec{v}_2 \hat{n} \times \vec{S}_1 \cdot \vec{v}_2 - 2 \vec{v}_2 \cdot \vec{v}_2 \hat{n} \times \vec{S}_1 \cdot \vec{v}_1 + 4 \vec{v}_2 \cdot \vec{v}_2 \hat{n} \times \vec{S}_1 \cdot \vec{v}_2 \right) \}$$

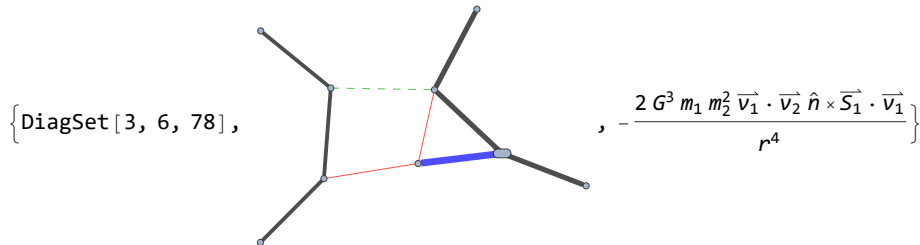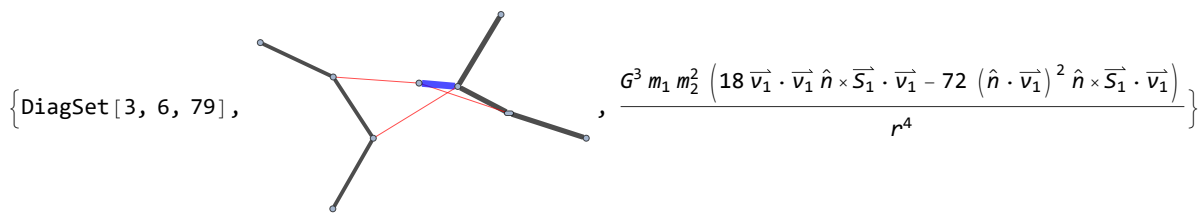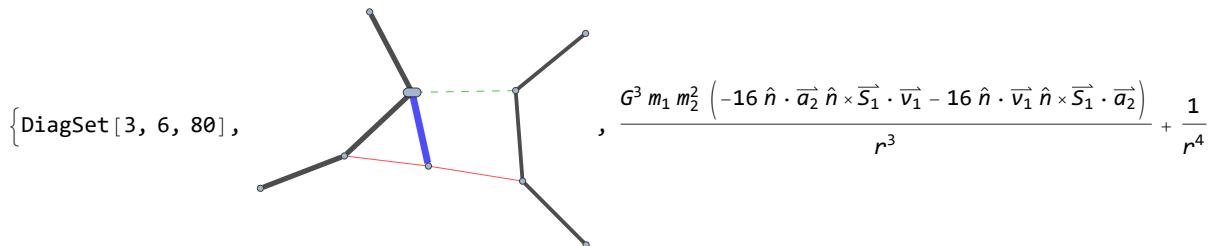

$$G^3 m_1 m_2^2 \left( -36 \left( \hat{n} \cdot \vec{v}_1 \right)^2 \hat{n} \times \vec{S}_1 \cdot \vec{v}_2 - 22 \hat{n} \cdot \vec{v}_1 \vec{S}_1 \times \vec{v}_1 \cdot \vec{v}_2 + 12 \hat{n} \cdot \vec{v}_2 \hat{n} \cdot \vec{v}_1 \hat{n} \times \vec{S}_1 \cdot \vec{v}_1 + 64 \hat{n} \cdot \vec{v}_2 \hat{n} \cdot \vec{v}_1 \hat{n} \times \vec{S}_1 \cdot \vec{v}_2 - \right. \\ \left. 16 \left( \hat{n} \cdot \vec{v}_2 \right)^2 \hat{n} \times \vec{S}_1 \cdot \vec{v}_1 + 16 \hat{n} \cdot \vec{v}_2 \vec{S}_1 \times \vec{v}_1 \cdot \vec{v}_2 + 10 \vec{v}_1 \cdot \vec{v}_1 \hat{n} \times \vec{S}_1 \cdot \vec{v}_2 - 12 \vec{v}_1 \cdot \vec{v}_2 \hat{n} \times \vec{S}_1 \cdot \vec{v}_1 - 24 \vec{v}_1 \cdot \vec{v}_2 \hat{n} \times \vec{S}_1 \cdot \vec{v}_2 \right) \}$$

$\{\text{DiagSet}[3, 6, 81],$ 
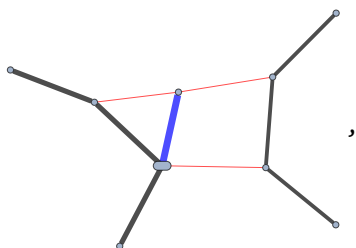
 $,$ 

$$\frac{G^3 m_1 m_2^2 \left( -8 \hat{n} \cdot \vec{a}_1 \hat{n} \times \vec{S}_1 \cdot \vec{v}_1 + 8 \hat{n} \cdot \vec{v}_1 \hat{n} \times \vec{S}_1 \cdot \vec{a}_1 + 8 \vec{S}_1 \times \vec{v}_1 \cdot \vec{a}_1 \right)}{r^3} + \frac{1}{r^4} G^3 m_1 m_2^2 \left( 72 (\hat{n} \cdot \vec{v}_1)^2 \hat{n} \times \vec{S}_1 \cdot \vec{v}_1 + \right. \\ \left. 24 \hat{n} \cdot \vec{v}_1 \vec{S}_1 \times \vec{v}_1 \cdot \vec{v}_2 - 96 \hat{n} \cdot \vec{v}_2 \hat{n} \cdot \vec{v}_1 \hat{n} \times \vec{S}_1 \cdot \vec{v}_1 + \vec{v}_1 \cdot \vec{v}_1 \hat{n} \times \vec{S}_1 \cdot \vec{v}_1 + 24 \vec{v}_1 \cdot \vec{v}_2 \hat{n} \times \vec{S}_1 \cdot \vec{v}_1 + 24 \vec{v}_2 \cdot \vec{v}_2 \hat{n} \times \vec{S}_1 \cdot \vec{v}_1 \right) \}$$

 $\{\text{DiagSet}[3, 6, 82],$ 
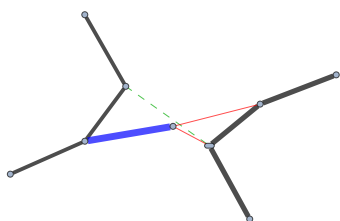
 $,$ 

$$\frac{G^3 m_1 m_2^2 \left( 8 (\hat{n} \cdot \vec{v}_2)^2 \hat{n} \times \vec{S}_1 \cdot \vec{v}_2 - 8 \vec{v}_2 \cdot \vec{v}_2 \hat{n} \times \vec{S}_1 \cdot \vec{v}_2 \right)}{r^4} \}$$

 $\{\text{DiagSet}[3, 6, 83],$ 
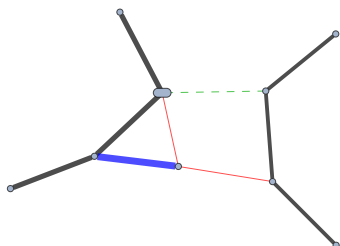
 $,$ 

$$\frac{G^3 m_1 m_2^2 \left( 16 \vec{v}_1 \cdot \vec{v}_1 \hat{n} \times \vec{S}_1 \cdot \vec{v}_2 - 32 (\hat{n} \cdot \vec{v}_1)^2 \hat{n} \times \vec{S}_1 \cdot \vec{v}_2 \right)}{r^4} \}$$

 $\{\text{DiagSet}[3, 6, 84],$ 
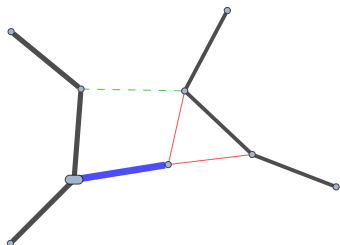
 $,$ 

$$-\frac{4 G^3 m_1 m_2^2 \vec{v}_1 \cdot \vec{v}_2 \hat{n} \times \vec{S}_1 \cdot \vec{v}_1}{r^4} \}$$

 $\{\text{DiagSet}[3, 6, 85],$ 
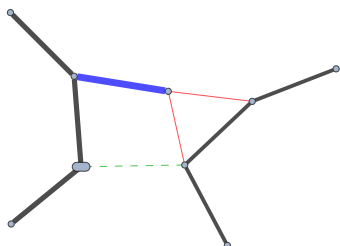
 $,$ 

$$\frac{G^3 m_1 m_2^2 \left( 2 (\hat{n} \cdot \vec{v}_1)^2 \hat{n} \times \vec{S}_1 \cdot \vec{v}_2 - 2 \vec{v}_1 \cdot \vec{v}_1 \hat{n} \times \vec{S}_1 \cdot \vec{v}_2 \right)}{r^4} \}$$

 $\{\text{DiagSet}[3, 6, 86],$ 
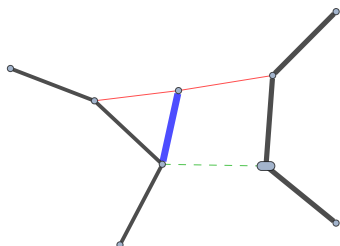
 $,$ 

$$\frac{G^3 m_1 m_2^2 \left( 8 (\hat{n} \cdot \vec{v}_2)^2 \hat{n} \times \vec{S}_1 \cdot \vec{v}_2 - 4 \vec{v}_2 \cdot \vec{v}_2 \hat{n} \times \vec{S}_1 \cdot \vec{v}_2 \right)}{r^4} \}$$

{DiagSet[3, 6, 87],

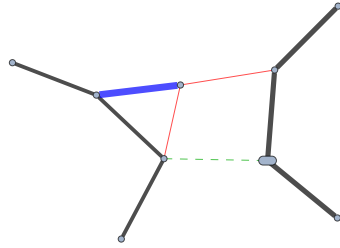

$$, \frac{G^3 m_1 m_2^2 \left( 4 \vec{v}_2 \cdot \vec{v}_2 \hat{n} \times \vec{S}_1 \cdot \vec{v}_2 - 8 (\hat{n} \cdot \vec{v}_2)^2 \hat{n} \times \vec{S}_1 \cdot \vec{v}_2 \right)}{r^4} \}$$

{DiagSet[3, 6, 88],

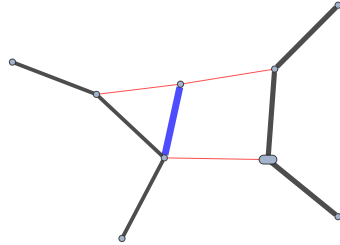

$$, \frac{G^3 m_1 m_2^2 \left( 12 \vec{v}_2 \cdot \vec{v}_2 \hat{n} \times \vec{S}_1 \cdot \vec{v}_1 - 24 (\hat{n} \cdot \vec{v}_2)^2 \hat{n} \times \vec{S}_1 \cdot \vec{v}_1 \right)}{r^4} \}$$

{DiagSet[3, 6, 89],

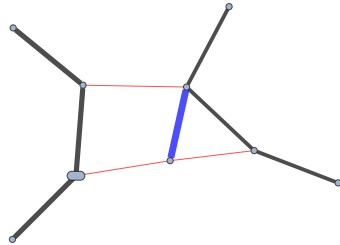

,

$$\frac{G^3 m_1 m_2^2 \left( -96 (\hat{n} \cdot \vec{v}_2)^2 \hat{n} \times \vec{S}_1 \cdot \vec{v}_1 + 48 \hat{n} \cdot \vec{v}_2 \vec{S}_1 \times \vec{v}_1 \cdot \vec{v}_2 + 24 \vec{v}_2 \cdot \vec{v}_2 \hat{n} \times \vec{S}_1 \cdot \vec{v}_1 \right)}{r^4} \}$$

{DiagSet[3, 6, 90],

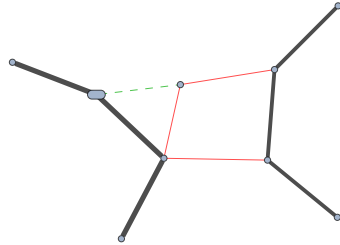

,

$$\frac{1}{r^3} G^3 m_1 m_2^2 \left( 8 \hat{n} \cdot \vec{v}_1 \hat{n} \times \vec{S}_1 \cdot \vec{a}_1 - 2 \vec{S}_1 \times \vec{a}_1 \cdot \vec{v}_2 + 2 \vec{S}_1 \times \vec{v}_1 \cdot \vec{a}_1 + 8 \hat{n} \cdot \vec{v}_1 \hat{n} \times \vec{S}_1 \cdot \vec{v}_1 - 2 \vec{S}_1 \times \vec{v}_1 \cdot \vec{v}_2 \right) + \frac{1}{r^4} G^3 m_1 m_2^2 \left( -8 (\hat{n} \cdot \vec{v}_1)^2 \hat{n} \times \vec{S}_1 \cdot \vec{v}_1 + \hat{n} \cdot \vec{v}_1 \vec{S}_1 \times \vec{v}_1 \cdot \vec{v}_2 + \frac{7}{2} \vec{v}_1 \cdot \vec{v}_1 \hat{n} \times \vec{S}_1 \cdot \vec{v}_1 + \vec{v}_1 \cdot \vec{v}_2 \hat{n} \times \vec{S}_1 \cdot \vec{v}_1 - \frac{3}{2} \vec{v}_2 \cdot \vec{v}_2 \hat{n} \times \vec{S}_1 \cdot \vec{v}_1 \right) \}$$

{DiagSet[3, 6, 91],

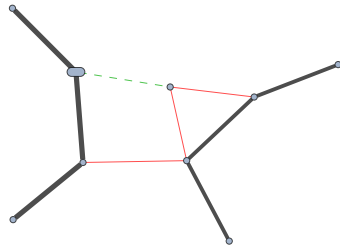

,

$$\frac{1}{r^3} G^3 m_1 m_2^2 \left( -2 \hat{n} \cdot \vec{v}_1 \hat{n} \times \vec{a}_1 \cdot \vec{S}_1 + 4 \hat{n} \cdot \vec{v}_2 \hat{n} \times \vec{a}_1 \cdot \vec{S}_1 - 2 \vec{a}_1 \times \vec{S}_1 \cdot \vec{v}_2 + 2 \hat{n} \cdot \vec{v}_1 \hat{n} \times \vec{S}_1 \cdot \vec{v}_1 - 4 \hat{n} \cdot \vec{v}_2 \hat{n} \times \vec{S}_1 \cdot \vec{v}_1 + 2 \vec{S}_1 \times \vec{v}_1 \cdot \vec{v}_2 \right) + \frac{1}{r^4} G^3 m_1 m_2^2 \left( -4 (\hat{n} \cdot \vec{v}_1)^2 \hat{n} \times \vec{S}_1 \cdot \vec{v}_1 - \frac{5}{2} \hat{n} \cdot \vec{v}_1 \vec{S}_1 \times \vec{v}_1 \cdot \vec{v}_2 + \right.$$

$$12 \hat{n} \cdot \vec{v}_2 \hat{n} \cdot \vec{v}_1 \hat{n} \times \vec{S}_1 \cdot \vec{v}_1 - \frac{3}{2} \vec{v}_1 \cdot \vec{v}_1 \hat{n} \times \vec{S}_1 \cdot \vec{v}_2 - \frac{7}{2} \vec{v}_1 \cdot \vec{v}_2 \hat{n} \times \vec{S}_1 \cdot \vec{v}_1 + 3 \vec{v}_2 \cdot \vec{v}_2 \hat{n} \times \vec{S}_1 \cdot \vec{v}_2 \Big\}$$

{DiagSet[3, 6, 92], 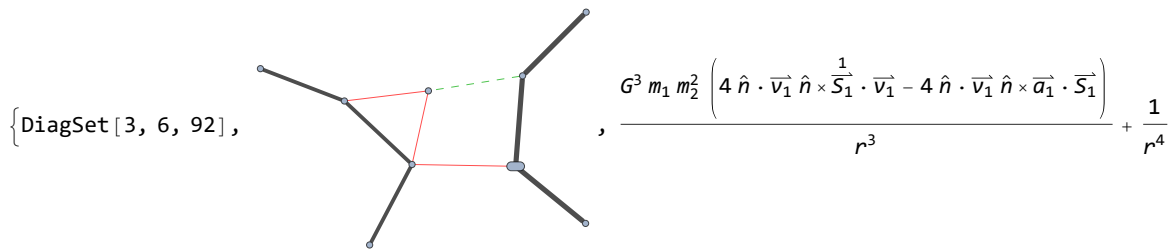

$$, \frac{G^3 m_1 m_2^2 \left( 4 \hat{n} \cdot \vec{v}_1 \hat{n} \times \vec{S}_1 \cdot \vec{v}_1 - 4 \hat{n} \cdot \vec{v}_1 \hat{n} \times \vec{a}_1 \cdot \vec{S}_1 \right)}{r^3} + \frac{1}{r^4}$$

$$G^3 m_1 m_2^2 \left( -12 (\hat{n} \cdot \vec{v}_1)^2 \hat{n} \times \vec{S}_1 \cdot \vec{v}_1 - 4 \hat{n} \cdot \vec{v}_1 \vec{S}_1 \times \vec{v}_1 \cdot \vec{v}_2 + 16 \hat{n} \cdot \vec{v}_2 \hat{n} \cdot \vec{v}_1 \hat{n} \times \vec{S}_1 \cdot \vec{v}_1 - 4 \vec{v}_1 \cdot \vec{v}_2 \hat{n} \times \vec{S}_1 \cdot \vec{v}_1 \right) \Big\}$$

{DiagSet[3, 6, 93], 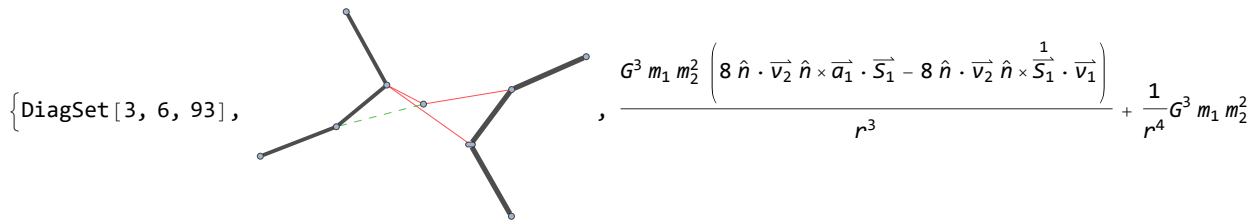

$$, \frac{G^3 m_1 m_2^2 \left( 8 \hat{n} \cdot \vec{v}_2 \hat{n} \times \vec{a}_1 \cdot \vec{S}_1 - 8 \hat{n} \cdot \vec{v}_2 \hat{n} \times \vec{S}_1 \cdot \vec{v}_1 \right)}{r^3} + \frac{1}{r^4} G^3 m_1 m_2^2$$

$$\left( -32 (\hat{n} \cdot \vec{v}_2)^2 \hat{n} \times \vec{S}_1 \cdot \vec{v}_1 + 8 \hat{n} \cdot \vec{v}_2 \vec{S}_1 \times \vec{v}_1 \cdot \vec{v}_2 + 16 \hat{n} \cdot \vec{v}_1 \hat{n} \cdot \vec{v}_2 \hat{n} \times \vec{S}_1 \cdot \vec{v}_1 + 4 \vec{v}_1 \cdot \vec{v}_2 \hat{n} \times \vec{S}_1 \cdot \vec{v}_1 + 4 \vec{v}_2 \cdot \vec{v}_2 \hat{n} \times \vec{S}_1 \cdot \vec{v}_1 \right) \Big\}$$

{DiagSet[3, 6, 94], 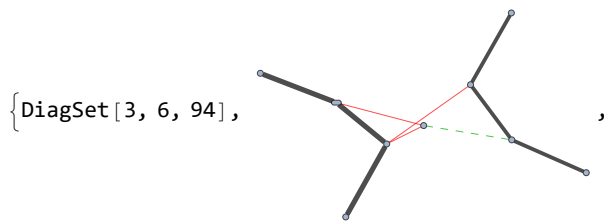

$$\frac{G^3 m_1 m_2^2 \left( -2 \hat{n} \cdot \vec{v}_2 \hat{n} \times \vec{S}_1 \cdot \vec{a}_1 + 2 \vec{S}_1 \times \vec{a}_1 \cdot \vec{v}_2 - 2 \hat{n} \cdot \vec{v}_2 \hat{n} \times \vec{S}_1 \cdot \vec{v}_1 + 2 \vec{S}_1 \times \vec{v}_1 \cdot \vec{v}_2 \right)}{r^3} + \frac{1}{r^4} G^3 m_1 m_2^2$$

$$\left( -6 (\hat{n} \cdot \vec{v}_2)^2 \hat{n} \times \vec{S}_1 \cdot \vec{v}_1 + 2 \hat{n} \cdot \vec{v}_2 \vec{S}_1 \times \vec{v}_1 \cdot \vec{v}_2 + 14 \hat{n} \cdot \vec{v}_1 \hat{n} \cdot \vec{v}_2 \hat{n} \times \vec{S}_1 \cdot \vec{v}_1 - 4 \hat{n} \cdot \vec{v}_1 \vec{S}_1 \times \vec{v}_1 \cdot \vec{v}_2 - 4 \vec{v}_1 \cdot \vec{v}_2 \hat{n} \times \vec{S}_1 \cdot \vec{v}_1 \right) \Big\}$$

{DiagSet[3, 6, 95], 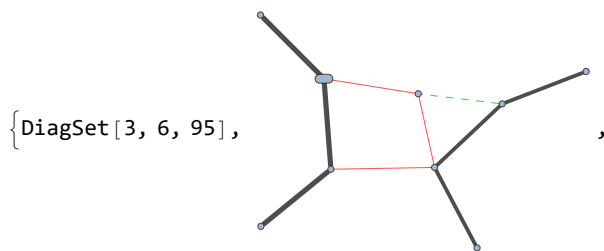

$$\frac{G^3 m_1 m_2^2 \left( -8 \hat{n} \cdot \vec{v}_2 \hat{n} \times \vec{a}_1 \cdot \vec{S}_1 + 4 \vec{a}_1 \times \vec{S}_1 \cdot \vec{v}_2 + 8 \hat{n} \cdot \vec{v}_2 \hat{n} \times \vec{S}_1 \cdot \vec{v}_1 - 4 \vec{S}_1 \times \vec{v}_1 \cdot \vec{v}_2 \right)}{r^3} + \frac{1}{r^4} G^3 m_1 m_2^2$$

$$\left( -48 (\hat{n} \cdot \vec{v}_2)^2 \hat{n} \times \vec{S}_1 \cdot \vec{v}_1 + 24 \hat{n} \cdot \vec{v}_2 \vec{S}_1 \times \vec{v}_1 \cdot \vec{v}_2 - 16 \hat{n} \cdot \vec{v}_1 \hat{n} \cdot \vec{v}_2 \hat{n} \times \vec{S}_1 \cdot \vec{v}_1 + 8 \vec{v}_1 \cdot \vec{v}_2 \hat{n} \times \vec{S}_1 \cdot \vec{v}_1 + 8 \vec{v}_2 \cdot \vec{v}_2 \hat{n} \times \vec{S}_1 \cdot \vec{v}_1 \right) \Big\}$$



{DiagSet[3, 6, 96],

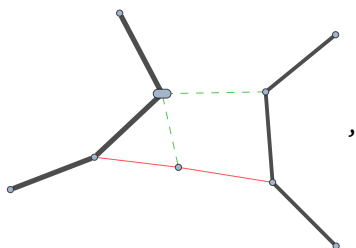

,

$$\frac{1}{r^3} G^3 m_1 m_2^2 \left( -8 \hat{n} \cdot \vec{a}_1 \hat{n} \times \vec{S}_1 \cdot \vec{v}_2 - 8 \hat{n} \cdot \vec{a}_2 \hat{n} \times \vec{S}_1 \cdot \vec{v}_2 + 8 \hat{n} \cdot \vec{v}_1 \hat{n} \times \vec{S}_1 \cdot \vec{a}_2 + \right. \\ \left. 8 \hat{n} \cdot \vec{v}_2 \hat{n} \times \vec{S}_1 \cdot \vec{a}_2 - 4 \vec{S}_1 \times \vec{a}_1 \cdot \vec{v}_2 + 4 \vec{S}_1 \times \vec{v}_1 \cdot \vec{a}_2 + 8 \vec{S}_1 \times \vec{v}_2 \cdot \vec{a}_2 \right) + \frac{1}{r^4} \\ G^3 m_1 m_2^2 \left( 32 (\hat{n} \cdot \vec{v}_1)^2 \hat{n} \times \vec{S}_1 \cdot \vec{v}_2 + 12 \hat{n} \cdot \vec{v}_1 \vec{S}_1 \times \vec{v}_1 \cdot \vec{v}_2 + 8 \hat{n} \cdot \vec{v}_2 \hat{n} \cdot \vec{v}_1 \hat{n} \times \vec{S}_1 \cdot \vec{v}_2 - 24 (\hat{n} \cdot \vec{v}_2)^2 \hat{n} \times \vec{S}_1 \cdot \vec{v}_2 - \right. \\ \left. 8 \vec{v}_1 \cdot \vec{v}_1 \hat{n} \times \vec{S}_1 \cdot \vec{v}_2 + 2 \vec{v}_1 \cdot \vec{v}_2 \hat{n} \times \vec{S}_1 \cdot \vec{v}_1 - 2 \vec{v}_1 \cdot \vec{v}_2 \hat{n} \times \vec{S}_1 \cdot \vec{v}_2 + 8 \vec{v}_2 \cdot \vec{v}_2 \hat{n} \times \vec{S}_1 \cdot \vec{v}_2 \right) \Big\}$$

{DiagSet[3, 6, 97],

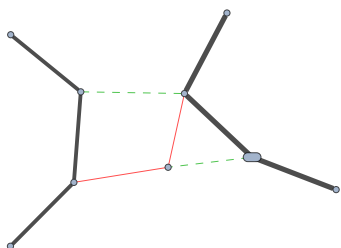

$$\left. , \frac{2 G^3 m_1 m_2^2 \vec{v}_1 \cdot \vec{v}_2 \hat{n} \times \vec{S}_1 \cdot \vec{v}_1}{r^4} \right\}$$

{DiagSet[3, 6, 98],

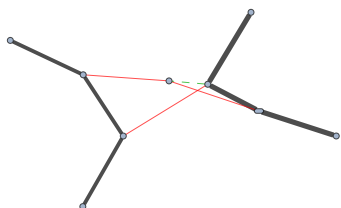

,

$$\frac{G^3 m_1 m_2^2 \left( 8 \hat{n} \cdot \vec{v}_1 \hat{n} \times \vec{S}_1 \cdot \vec{a}_1 + 4 \vec{S}_1 \times \vec{v}_1 \cdot \vec{a}_1 + 8 \hat{n} \cdot \vec{v}_1 \hat{n} \times \vec{S}_1 \cdot \vec{v}_1 \right)}{r^3} + \frac{1}{r^4} G^3 m_1 m_2^2 \\ \left( -24 (\hat{n} \cdot \vec{v}_1)^2 \hat{n} \times \vec{S}_1 \cdot \vec{v}_1 + 6 \hat{n} \cdot \vec{v}_1 \vec{S}_1 \times \vec{v}_1 \cdot \vec{v}_2 - 24 \hat{n} \cdot \vec{v}_2 \hat{n} \cdot \vec{v}_1 \hat{n} \times \vec{S}_1 \cdot \vec{v}_1 + 6 \vec{v}_1 \cdot \vec{v}_1 \hat{n} \times \vec{S}_1 \cdot \vec{v}_1 + 6 \vec{v}_1 \cdot \vec{v}_2 \hat{n} \times \vec{S}_1 \cdot \vec{v}_1 \right) \Big\}$$

{DiagSet[3, 6, 99],

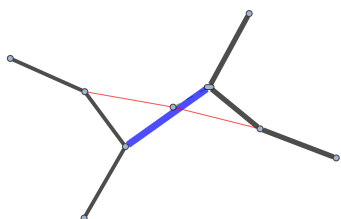

,

$$\frac{G^3 m_1 m_2^2 \left( \hat{n} \cdot \vec{v}_2 \left( -(\vec{S}_1 \times \vec{v}_1 \cdot \vec{v}_2) \right) - \vec{v}_1 \cdot \vec{v}_2 \hat{n} \times \vec{S}_1 \cdot \vec{v}_2 + 2 \vec{v}_2 \cdot \vec{v}_2 \hat{n} \times \vec{S}_1 \cdot \vec{v}_1 \right)}{r^4} \Big\}$$

{DiagSet[3, 6, 100],

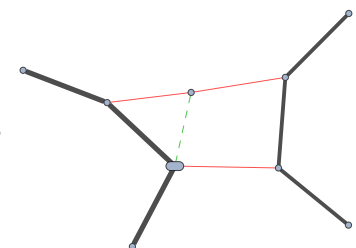

$$\left. , \frac{1}{r^4} \right\}$$

$$G^3 m_1 m_2^2 \left( -8 (\hat{n} \cdot \vec{v}_2)^2 \hat{n} \times \vec{S}_1 \cdot \vec{v}_1 + 4 \hat{n} \cdot \vec{v}_2 \vec{S}_1 \times \vec{v}_1 \cdot \vec{v}_2 - 8 \hat{n} \cdot \vec{v}_1 \hat{n} \cdot \vec{v}_2 \hat{n} \times \vec{S}_1 \cdot \vec{v}_1 - 3 \vec{v}_1 \cdot \vec{v}_1 \hat{n} \times \vec{S}_1 \cdot \vec{v}_1 - 6 \vec{v}_2 \cdot \vec{v}_2 \hat{n} \times \vec{S}_1 \cdot \vec{v}_1 \right) \Big\}$$

$\{\text{DiagSet}[3, 6, 101],$ 
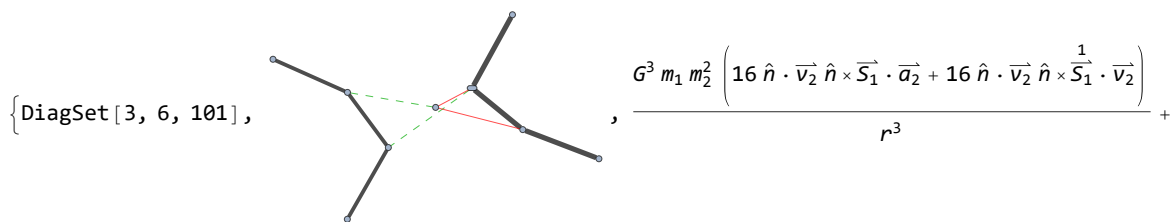
 $, \frac{G^3 m_1 m_2^2 \left( 16 \hat{n} \cdot \vec{v}_2 \hat{n} \times \vec{S}_1 \cdot \vec{a}_2 + 16 \hat{n} \cdot \vec{v}_2 \hat{n} \times \vec{S}_1 \cdot \vec{v}_2 \right)}{r^3} +$

$$\frac{1}{r^4} G^3 m_1 m_2^2 \left( 48 (\hat{n} \cdot \vec{v}_2)^2 \hat{n} \times \vec{S}_1 \cdot \vec{v}_2 - 16 \hat{n} \cdot \vec{v}_2 \vec{S}_1 \times \vec{v}_1 \cdot \vec{v}_2 - 64 \hat{n} \cdot \vec{v}_1 \hat{n} \cdot \vec{v}_2 \hat{n} \times \vec{S}_1 \cdot \vec{v}_2 + 16 \vec{v}_1 \cdot \vec{v}_2 \hat{n} \times \vec{S}_1 \cdot \vec{v}_2 \right) \Big\}$$

$\{\text{DiagSet}[3, 6, 102],$ 
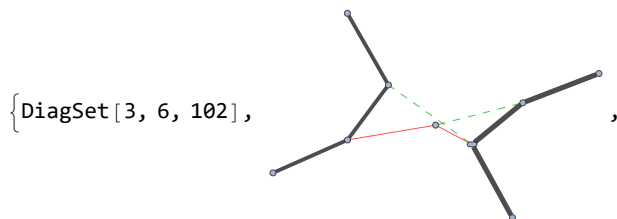
 $,$

$$\frac{G^3 m_1 m_2^2 \left( -32 \hat{n} \cdot \vec{v}_1 \hat{n} \times \vec{S}_1 \cdot \vec{a}_2 - 32 \hat{n} \cdot \vec{v}_1 \hat{n} \times \vec{S}_1 \cdot \vec{v}_2 \right)}{r^3} + \frac{1}{r^4} G^3 m_1 m_2^2 \left( 128 (\hat{n} \cdot \vec{v}_1)^2 \hat{n} \times \vec{S}_1 \cdot \vec{v}_2 + 32 \hat{n} \cdot \vec{v}_1 \vec{S}_1 \times \vec{v}_1 \cdot \vec{v}_2 - 64 \hat{n} \cdot \vec{v}_2 \hat{n} \cdot \vec{v}_1 \hat{n} \times \vec{S}_1 \cdot \vec{v}_2 - 16 \vec{v}_1 \cdot \vec{v}_1 \hat{n} \times \vec{S}_1 \cdot \vec{v}_2 - 16 \vec{v}_1 \cdot \vec{v}_2 \hat{n} \times \vec{S}_1 \cdot \vec{v}_2 \right) \Big\}$$

$\{\text{DiagSet}[3, 6, 103],$ 
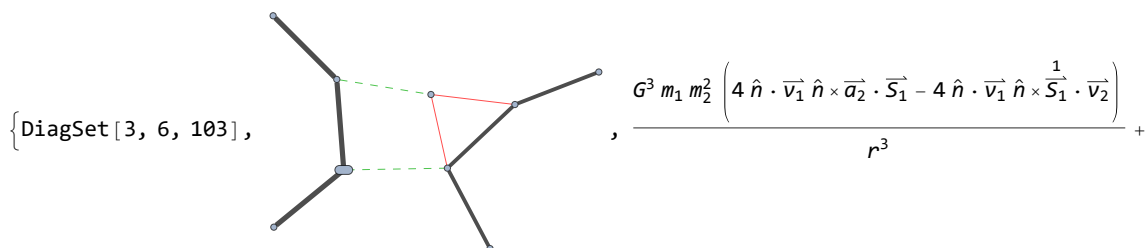
 $, \frac{G^3 m_1 m_2^2 \left( 4 \hat{n} \cdot \vec{v}_1 \hat{n} \times \vec{a}_2 \cdot \vec{S}_1 - 4 \hat{n} \cdot \vec{v}_1 \hat{n} \times \vec{S}_1 \cdot \vec{v}_2 \right)}{r^3} +$

$$\frac{1}{r^4} G^3 m_1 m_2^2 \left( 12 (\hat{n} \cdot \vec{v}_1)^2 \hat{n} \times \vec{S}_1 \cdot \vec{v}_2 + 4 \hat{n} \cdot \vec{v}_1 \vec{S}_1 \times \vec{v}_1 \cdot \vec{v}_2 - 16 \hat{n} \cdot \vec{v}_2 \hat{n} \cdot \vec{v}_1 \hat{n} \times \vec{S}_1 \cdot \vec{v}_2 + 4 \vec{v}_1 \cdot \vec{v}_2 \hat{n} \times \vec{S}_1 \cdot \vec{v}_2 \right) \Big\}$$

$\{\text{DiagSet}[3, 6, 104],$ 
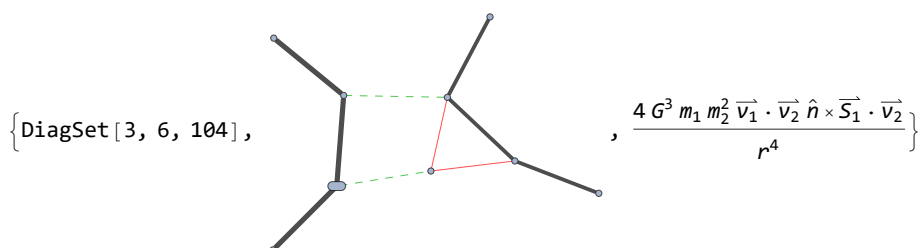
 $, \frac{4 G^3 m_1 m_2^2 \vec{v}_1 \cdot \vec{v}_2 \hat{n} \times \vec{S}_1 \cdot \vec{v}_2}{r^4} \Big\}$

$\{\text{DiagSet}[3, 6, 105],$ 
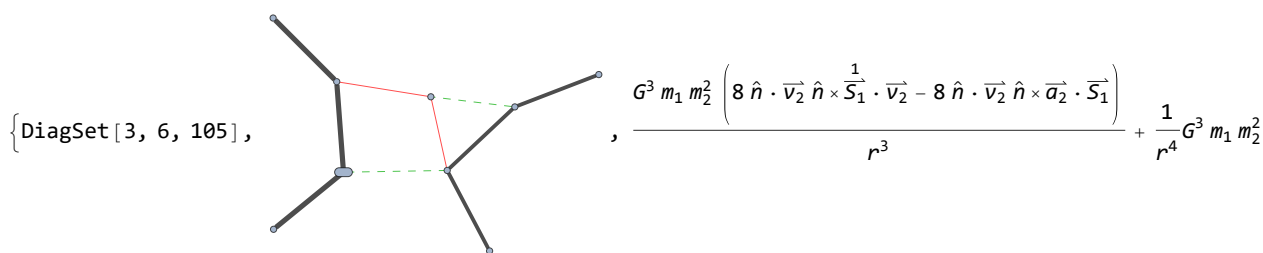
 $, \frac{G^3 m_1 m_2^2 \left( 8 \hat{n} \cdot \vec{v}_2 \hat{n} \times \vec{S}_1 \cdot \vec{v}_2 - 8 \hat{n} \cdot \vec{v}_2 \hat{n} \times \vec{a}_2 \cdot \vec{S}_1 \right)}{r^3} + \frac{1}{r^4} G^3 m_1 m_2^2$

$$\left( 32 (\hat{n} \cdot \vec{v}_2)^2 \hat{n} \times \vec{S}_1 \cdot \vec{v}_2 - 8 \hat{n} \cdot \vec{v}_2 \vec{S}_1 \times \vec{v}_1 \cdot \vec{v}_2 - 16 \hat{n} \cdot \vec{v}_1 \hat{n} \cdot \vec{v}_2 \hat{n} \times \vec{S}_1 \cdot \vec{v}_2 - 4 \vec{v}_1 \cdot \vec{v}_2 \hat{n} \times \vec{S}_1 \cdot \vec{v}_2 - 4 \vec{v}_2 \cdot \vec{v}_2 \hat{n} \times \vec{S}_1 \cdot \vec{v}_2 \right) \Big\}$$

{DiagSet[3, 6, 106],

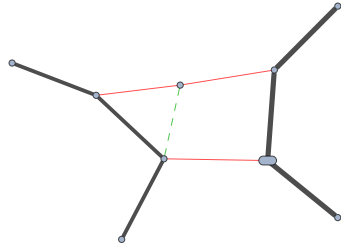

,  $\frac{1}{r^4}$

$$G^3 m_1 m_2^2 \left( -8 (\hat{n} \cdot \vec{v}_2)^2 \hat{n} \times \vec{S}_1 \cdot \vec{v}_1 - 8 \hat{n} \cdot \vec{v}_1 \hat{n} \cdot \vec{v}_2 \hat{n} \times \vec{S}_1 \cdot \vec{v}_1 + 4 \vec{v}_1 \cdot \vec{v}_2 \hat{n} \times \vec{S}_1 \cdot \vec{v}_1 + 4 \vec{v}_2 \cdot \vec{v}_2 \hat{n} \times \vec{S}_1 \cdot \vec{v}_1 \right) \}$$

{DiagSet[3, 6, 107],

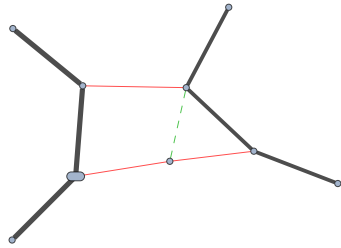

,

$$G^3 m_1 m_2^2 \left( -8 \hat{n} \cdot \vec{v}_2 \hat{n} \times \vec{a}_1 \cdot \vec{S}_1 + 4 \vec{a}_1 \times \vec{S}_1 \cdot \vec{v}_2 + 8 \hat{n} \cdot \vec{v}_2 \hat{n} \times \vec{S}_1 \cdot \vec{v}_1 - 4 \vec{S}_1 \times \vec{v}_1 \cdot \vec{v}_2 \right) \frac{1}{r^3} +$$

$$\frac{1}{r^4} G^3 m_1 m_2^2 \left( -32 (\hat{n} \cdot \vec{v}_2)^2 \hat{n} \times \vec{S}_1 \cdot \vec{v}_1 + 16 \hat{n} \cdot \vec{v}_2 \vec{S}_1 \times \vec{v}_1 \cdot \vec{v}_2 - 32 \hat{n} \cdot \vec{v}_1 \hat{n} \cdot \vec{v}_2 \hat{n} \times \vec{S}_1 \cdot \vec{v}_1 + 8 \hat{n} \cdot \vec{v}_1 \vec{S}_1 \times \vec{v}_1 \cdot \vec{v}_2 + 8 \vec{v}_1 \cdot \vec{v}_2 \hat{n} \times \vec{S}_1 \cdot \vec{v}_1 + 8 \vec{v}_2 \cdot \vec{v}_2 \hat{n} \times \vec{S}_1 \cdot \vec{v}_1 \right) \}$$

{DiagSet[3, 6, 108],

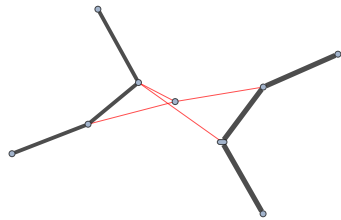

,

$$\frac{1}{r^3} G^3 m_1 m_2^2 \left( -8 \hat{n} \cdot \vec{v}_1 \hat{n} \times \vec{a}_1 \cdot \vec{S}_1 + 4 \hat{n} \cdot \vec{v}_2 \hat{n} \times \vec{a}_1 \cdot \vec{S}_1 + 8 \hat{n} \cdot \vec{v}_1 \hat{n} \times \vec{S}_1 \cdot \vec{v}_1 - 4 \hat{n} \cdot \vec{v}_2 \hat{n} \times \vec{S}_1 \cdot \vec{v}_1 \right) +$$

$$\frac{1}{r^4} G^3 m_1 m_2^2 \left( -24 (\hat{n} \cdot \vec{v}_1)^2 \hat{n} \times \vec{S}_1 \cdot \vec{v}_1 - 8 \hat{n} \cdot \vec{v}_1 \vec{S}_1 \times \vec{v}_1 \cdot \vec{v}_2 + 52 \hat{n} \cdot \vec{v}_2 \hat{n} \cdot \vec{v}_1 \hat{n} \times \vec{S}_1 \cdot \vec{v}_1 - 14 (\hat{n} \cdot \vec{v}_2)^2 \hat{n} \times \vec{S}_1 \cdot \vec{v}_1 + 4 \hat{n} \cdot \vec{v}_2 \vec{S}_1 \times \vec{v}_1 \cdot \vec{v}_2 - 8 \vec{v}_1 \cdot \vec{v}_2 \hat{n} \times \vec{S}_1 \cdot \vec{v}_1 + 2 \vec{v}_2 \cdot \vec{v}_2 \hat{n} \times \vec{S}_1 \cdot \vec{v}_1 \right) \}$$

{DiagSet[3, 6, 109],

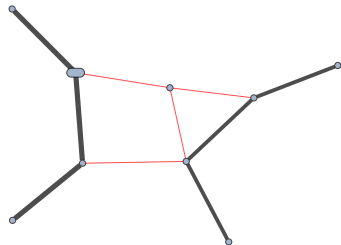

,  $\frac{1}{r^3} G^3 m_1 m_2^2$

$$\left( -8 \hat{n} \cdot \vec{v}_1 \hat{n} \times \vec{a}_1 \cdot \vec{S}_1 + 24 \hat{n} \cdot \vec{v}_2 \hat{n} \times \vec{a}_1 \cdot \vec{S}_1 - 8 \vec{a}_1 \times \vec{S}_1 \cdot \vec{v}_2 + 8 \hat{n} \cdot \vec{v}_1 \hat{n} \times \vec{S}_1 \cdot \vec{v}_1 - 24 \hat{n} \cdot \vec{v}_2 \hat{n} \times \vec{S}_1 \cdot \vec{v}_1 + 8 \vec{S}_1 \times \vec{v}_1 \cdot \vec{v}_2 \right) +$$

$$\frac{1}{r^4} G^3 m_1 m_2^2 \left( -16 (\hat{n} \cdot \vec{v}_1)^2 \hat{n} \times \vec{S}_1 \cdot \vec{v}_1 - 20 \hat{n} \cdot \vec{v}_1 \vec{S}_1 \times \vec{v}_1 \cdot \vec{v}_2 + 88 \hat{n} \cdot \vec{v}_2 \hat{n} \cdot \vec{v}_1 \hat{n} \times \vec{S}_1 \cdot \vec{v}_1 - 16 (\hat{n} \cdot \vec{v}_2)^2 \hat{n} \times \vec{S}_1 \cdot \vec{v}_1 + 8 \hat{n} \cdot \vec{v}_2 \vec{S}_1 \times \vec{v}_1 \cdot \vec{v}_2 - 16 \vec{v}_1 \cdot \vec{v}_2 \hat{n} \times \vec{S}_1 \cdot \vec{v}_1 + 4 \vec{v}_2 \cdot \vec{v}_2 \hat{n} \times \vec{S}_1 \cdot \vec{v}_1 \right) \}$$

{DiagSet[3, 6, 110],

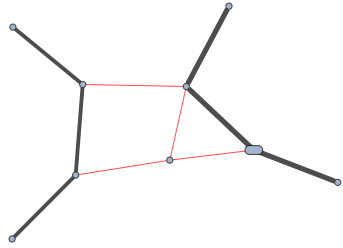

,

$$\frac{1}{r^3} G^3 m_1 m_2^2 \left( 6 \hat{n} \cdot \vec{v}_1 \hat{n} \times \vec{S}_1 \cdot \vec{a}_1 - 12 \hat{n} \cdot \vec{v}_2 \hat{n} \times \vec{S}_1 \cdot \vec{a}_1 + 4 \vec{S}_1 \times \vec{a}_1 \cdot \vec{v}_2 + \right. \\ \left. 2 \vec{S}_1 \times \vec{v}_1 \cdot \vec{a}_1 + 6 \hat{n} \cdot \vec{v}_1 \hat{n} \times \vec{S}_1 \cdot \vec{v}_1 - 12 \hat{n} \cdot \vec{v}_2 \hat{n} \times \vec{S}_1 \cdot \vec{v}_1 + 4 \vec{S}_1 \times \vec{v}_1 \cdot \vec{v}_2 \right) + \frac{1}{r^4} \\ G^3 m_1 m_2^2 \left( -10 (\hat{n} \cdot \vec{v}_1)^2 \hat{n} \times \vec{S}_1 \cdot \vec{v}_1 - 12 \hat{n} \cdot \vec{v}_1 \vec{S}_1 \times \vec{v}_1 \cdot \vec{v}_2 + 46 \hat{n} \cdot \vec{v}_2 \hat{n} \cdot \vec{v}_1 \hat{n} \times \vec{S}_1 \cdot \vec{v}_1 - 8 (\hat{n} \cdot \vec{v}_2)^2 \hat{n} \times \vec{S}_1 \cdot \vec{v}_1 + \right. \\ \left. 4 \hat{n} \cdot \vec{v}_2 \vec{S}_1 \times \vec{v}_1 \cdot \vec{v}_2 + 2 \vec{v}_1 \cdot \vec{v}_1 \hat{n} \times \vec{S}_1 \cdot \vec{v}_1 - 8 \vec{v}_1 \cdot \vec{v}_2 \hat{n} \times \vec{S}_1 \cdot \vec{v}_1 \right) \Big\}$$

{DiagSet[3, 6, 111],

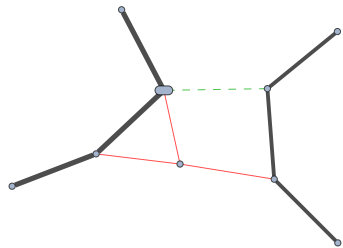

,

$$\frac{1}{r^3} G^3 m_1 m_2^2 \left( -16 \hat{n} \cdot \vec{v}_1 \hat{n} \times \vec{S}_1 \cdot \vec{a}_2 + 32 \hat{n} \cdot \vec{v}_2 \hat{n} \times \vec{S}_1 \cdot \vec{a}_2 - 16 \hat{n} \cdot \vec{v}_1 \hat{n} \times \vec{S}_1 \cdot \vec{v}_2 + 32 \hat{n} \cdot \vec{v}_2 \hat{n} \times \vec{S}_1 \cdot \vec{v}_2 \right) + \\ \frac{1}{r^4} G^3 m_1 m_2^2 \left( 56 (\hat{n} \cdot \vec{v}_1)^2 \hat{n} \times \vec{S}_1 \cdot \vec{v}_2 + 16 \hat{n} \cdot \vec{v}_1 \vec{S}_1 \times \vec{v}_1 \cdot \vec{v}_2 - 208 \hat{n} \cdot \vec{v}_2 \hat{n} \cdot \vec{v}_1 \hat{n} \times \vec{S}_1 \cdot \vec{v}_2 + \right. \\ \left. 96 (\hat{n} \cdot \vec{v}_2)^2 \hat{n} \times \vec{S}_1 \cdot \vec{v}_2 - 32 \hat{n} \cdot \vec{v}_2 \vec{S}_1 \times \vec{v}_1 \cdot \vec{v}_2 - 8 \vec{v}_1 \cdot \vec{v}_1 \hat{n} \times \vec{S}_1 \cdot \vec{v}_2 + 32 \vec{v}_1 \cdot \vec{v}_2 \hat{n} \times \vec{S}_1 \cdot \vec{v}_2 \right) \Big\}$$

{DiagSet[3, 6, 112],

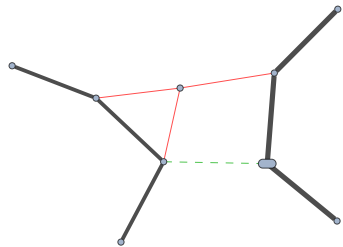

,

$$\frac{1}{r^3} G^3 m_1 m_2^2 \left( 8 \hat{n} \cdot \vec{v}_1 \hat{n} \times \vec{a}_2 \cdot \vec{S}_1 - 4 \hat{n} \cdot \vec{v}_2 \hat{n} \times \vec{a}_2 \cdot \vec{S}_1 - 8 \hat{n} \cdot \vec{v}_1 \hat{n} \times \vec{S}_1 \cdot \vec{v}_2 + 4 \hat{n} \cdot \vec{v}_2 \hat{n} \times \vec{S}_1 \cdot \vec{v}_2 \right) + \\ \frac{1}{r^4} G^3 m_1 m_2^2 \left( 24 (\hat{n} \cdot \vec{v}_1)^2 \hat{n} \times \vec{S}_1 \cdot \vec{v}_2 + 8 \hat{n} \cdot \vec{v}_1 \vec{S}_1 \times \vec{v}_1 \cdot \vec{v}_2 - 52 \hat{n} \cdot \vec{v}_2 \hat{n} \cdot \vec{v}_1 \hat{n} \times \vec{S}_1 \cdot \vec{v}_2 + \right. \\ \left. 14 (\hat{n} \cdot \vec{v}_2)^2 \hat{n} \times \vec{S}_1 \cdot \vec{v}_2 - 4 \hat{n} \cdot \vec{v}_2 \vec{S}_1 \times \vec{v}_1 \cdot \vec{v}_2 + 8 \vec{v}_1 \cdot \vec{v}_2 \hat{n} \times \vec{S}_1 \cdot \vec{v}_2 - 2 \vec{v}_2 \cdot \vec{v}_2 \hat{n} \times \vec{S}_1 \cdot \vec{v}_2 \right) \Big\}$$

{DiagSet[3, 6, 113],

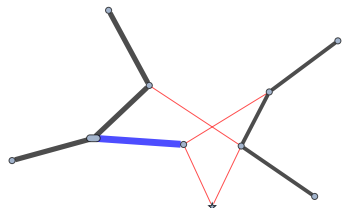

,

$$\frac{1}{r^3} G^3 m_1 m_2^2 \left( \frac{1}{2} \hat{n} \cdot \vec{a}_1 \hat{n} \times \vec{S}_1 \cdot \vec{v}_2 - \hat{n} \cdot \vec{v}_1 \hat{n} \times \vec{a}_1 \cdot \vec{S}_1 + \frac{3}{2} \hat{n} \cdot \vec{v}_2 \hat{n} \times \vec{a}_1 \cdot \vec{S}_1 - \right.$$

$$\frac{1}{2} \vec{a}_1 \times \vec{S}_1 \cdot \vec{v}_2 + \hat{n} \cdot \vec{v}_1 \hat{n} \times \vec{S}_1 \cdot \vec{v}_1 + \frac{1}{2} \hat{n} \cdot \vec{v}_1 \hat{n} \times \vec{S}_1 \cdot \vec{v}_2 - \frac{3}{2} \hat{n} \cdot \vec{v}_2 \hat{n} \times \vec{S}_1 \cdot \vec{v}_1 + \frac{1}{2} \vec{S}_1 \times \vec{v}_1 \cdot \vec{v}_2 \Big) +$$

$$\frac{1}{r^4} G^3 m_1 m_2^2 \left( -2 (\hat{n} \cdot \vec{v}_1)^2 \hat{n} \times \vec{S}_1 \cdot \vec{v}_1 - \frac{3}{2} (\hat{n} \cdot \vec{v}_1)^2 \hat{n} \times \vec{S}_1 \cdot \vec{v}_2 - 2 \hat{n} \cdot \vec{v}_1 \vec{S}_1 \times \vec{v}_1 \cdot \vec{v}_2 + \right.$$

$$\frac{11}{2} \hat{n} \cdot \vec{v}_2 \hat{n} \cdot \vec{v}_1 \hat{n} \times \vec{S}_1 \cdot \vec{v}_1 + \frac{3}{2} \hat{n} \cdot \vec{v}_2 \hat{n} \cdot \vec{v}_1 \hat{n} \times \vec{S}_1 \cdot \vec{v}_2 - \frac{5}{2} (\hat{n} \cdot \vec{v}_2)^2 \hat{n} \times \vec{S}_1 \cdot \vec{v}_1 +$$

$$\left. \frac{3}{2} \hat{n} \cdot \vec{v}_2 \vec{S}_1 \times \vec{v}_1 \cdot \vec{v}_2 + \frac{1}{2} \vec{v}_1 \cdot \vec{v}_1 \hat{n} \times \vec{S}_1 \cdot \vec{v}_2 - \frac{1}{2} \vec{v}_1 \cdot \vec{v}_2 \hat{n} \times \vec{S}_1 \cdot \vec{v}_1 + \frac{1}{2} \vec{v}_2 \cdot \vec{v}_2 \hat{n} \times \vec{S}_1 \cdot \vec{v}_1 \right\}$$

{DiagSet[3, 6, 114],

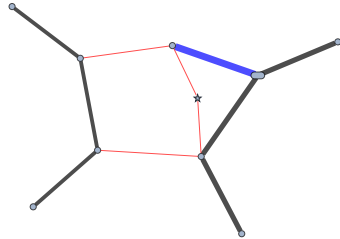

,  $\frac{1}{r^3} G^3 m_1 m_2^2$

$$\left( \frac{5}{4} \hat{n} \cdot \vec{a}_1 \hat{n} \times \vec{S}_1 \cdot \vec{v}_1 + \frac{3}{4} \hat{n} \cdot \vec{v}_1 \hat{n} \times \vec{S}_1 \cdot \vec{a}_1 - \frac{1}{2} \hat{n} \cdot \vec{v}_2 \hat{n} \times \vec{S}_1 \cdot \vec{a}_1 - \frac{1}{2} \vec{S}_1 \times \vec{v}_1 \cdot \vec{a}_1 + 2 \hat{n} \cdot \vec{v}_1 \hat{n} \times \vec{S}_1 \cdot \vec{v}_1 - \frac{1}{2} \hat{n} \cdot \vec{v}_2 \hat{n} \times \vec{S}_1 \cdot \vec{v}_1 \right) +$$

$$\frac{1}{r^4} G^3 m_1 m_2^2 \left( -2 (\hat{n} \cdot \vec{v}_1)^2 \hat{n} \times \vec{S}_1 \cdot \vec{v}_1 - 2 \hat{n} \cdot \vec{v}_1 \vec{S}_1 \times \vec{v}_1 \cdot \vec{v}_2 + \frac{13}{2} \hat{n} \cdot \vec{v}_2 \hat{n} \cdot \vec{v}_1 \hat{n} \times \vec{S}_1 \cdot \vec{v}_1 - \right.$$

$$\left. (\hat{n} \cdot \vec{v}_2)^2 \hat{n} \times \vec{S}_1 \cdot \vec{v}_1 + \frac{1}{2} \hat{n} \cdot \vec{v}_2 \vec{S}_1 \times \vec{v}_1 \cdot \vec{v}_2 + \vec{v}_1 \cdot \vec{v}_1 \hat{n} \times \vec{S}_1 \cdot \vec{v}_1 - \frac{3}{2} \vec{v}_1 \cdot \vec{v}_2 \hat{n} \times \vec{S}_1 \cdot \vec{v}_1 \right\}$$

{DiagSet[3, 6, 115],

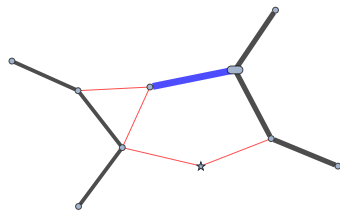

,  $\frac{G^3 m_1 m_2^2 \left( \frac{1}{2} \hat{n} \cdot \vec{v}_1 \hat{n} \times \vec{a}_1 \cdot \vec{S}_1 - \frac{1}{2} \hat{n} \cdot \vec{v}_1 \hat{n} \times \vec{S}_1 \cdot \vec{v}_1 \right)}{r^3} +$

$$\frac{1}{r^4} G^3 m_1 m_2^2 \left( 2 (\hat{n} \cdot \vec{v}_1)^2 \hat{n} \times \vec{S}_1 \cdot \vec{v}_1 + \frac{1}{2} \hat{n} \cdot \vec{v}_1 \vec{S}_1 \times \vec{v}_1 \cdot \vec{v}_2 - \frac{5}{2} \hat{n} \cdot \vec{v}_2 \hat{n} \cdot \vec{v}_1 \hat{n} \times \vec{S}_1 \cdot \vec{v}_1 + \frac{1}{2} \vec{v}_1 \cdot \vec{v}_2 \hat{n} \times \vec{S}_1 \cdot \vec{v}_1 \right\}$$

{DiagSet[3, 6, 116],

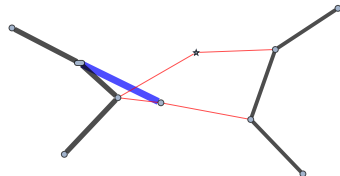

,  $\frac{G^3 m_1 m_2^2 \left( \frac{1}{4} \hat{n} \cdot \vec{v}_2 \hat{n} \times \vec{S}_1 \cdot \vec{a}_1 + \frac{1}{4} \hat{n} \cdot \vec{v}_2 \hat{n} \times \vec{S}_1 \cdot \vec{v}_1 \right)}{r^3} +$

$$\frac{1}{r^4} G^3 m_1 m_2^2 \left( (\hat{n} \cdot \vec{v}_2)^2 \hat{n} \times \vec{S}_1 \cdot \vec{v}_1 - \frac{1}{4} \hat{n} \cdot \vec{v}_2 \vec{S}_1 \times \vec{v}_1 \cdot \vec{v}_2 - \frac{5}{4} \hat{n} \cdot \vec{v}_1 \hat{n} \cdot \vec{v}_2 \hat{n} \times \vec{S}_1 \cdot \vec{v}_1 + \frac{1}{4} \vec{v}_1 \cdot \vec{v}_2 \hat{n} \times \vec{S}_1 \cdot \vec{v}_1 \right\}$$

{DiagSet[3, 6, 117],

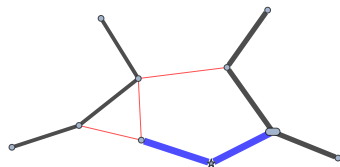

,  $\frac{1}{r^3} G^3 m_1 m_2^2$

$$\left( \frac{1}{2} \hat{n} \cdot \vec{v}_1 \hat{n} \times \vec{a}_1 \cdot \vec{S}_1 - \frac{3}{2} \hat{n} \cdot \vec{v}_2 \hat{n} \times \vec{a}_1 \cdot \vec{S}_1 + \frac{1}{2} \vec{a}_1 \times \vec{S}_1 \cdot \vec{v}_2 - \frac{1}{2} \hat{n} \cdot \vec{v}_1 \hat{n} \times \vec{S}_1 \cdot \vec{v}_1 + \frac{3}{2} \hat{n} \cdot \vec{v}_2 \hat{n} \times \vec{S}_1 \cdot \vec{v}_1 - \frac{1}{2} \vec{S}_1 \times \vec{v}_1 \cdot \vec{v}_2 \right) +$$

$$\frac{1}{r^4} G^3 m_1 m_2^2 \left( (\hat{n} \cdot \vec{v}_1)^2 \hat{n} \times \vec{S}_1 \cdot \vec{v}_1 + \hat{n} \cdot \vec{v}_1 \vec{S}_1 \times \vec{v}_1 \cdot \vec{v}_2 - 5 \hat{n} \cdot \vec{v}_2 \hat{n} \cdot \vec{v}_1 \hat{n} \times \vec{S}_1 \cdot \vec{v}_1 + \vec{v}_1 \cdot \vec{v}_2 \hat{n} \times \vec{S}_1 \cdot \vec{v}_1 \right\}$$

$\{\text{DiagSet}[3, 6, 118],$ 
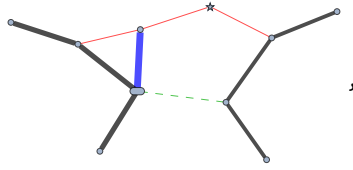
 $,$ 

$$\frac{1}{r^3} G^3 m_1 m_2^2 \left( \frac{4}{3} \hat{n} \cdot \vec{a}_2 \hat{n} \times \vec{S}_1 \cdot \vec{v}_2 + \frac{4}{3} \hat{n} \cdot \vec{v}_2 \hat{n} \times \vec{S}_1 \cdot \vec{a}_2 - \frac{4}{3} \vec{S}_1 \times \vec{v}_2 \cdot \vec{a}_2 + \frac{8}{3} \hat{n} \cdot \vec{v}_2 \hat{n} \times \vec{S}_1 \cdot \vec{v}_2 \right) + \frac{1}{r^4} G^3 m_1 m_2^2 \left( 8 (\hat{n} \cdot \vec{v}_2)^2 \hat{n} \times \vec{S}_1 \cdot \vec{v}_2 - \frac{8}{3} \hat{n} \cdot \vec{v}_2 \vec{S}_1 \times \vec{v}_1 \cdot \vec{v}_2 - \frac{40}{3} \hat{n} \cdot \vec{v}_1 \hat{n} \cdot \vec{v}_2 \hat{n} \times \vec{S}_1 \cdot \vec{v}_2 + \frac{8}{3} \vec{v}_1 \cdot \vec{v}_2 \hat{n} \times \vec{S}_1 \cdot \vec{v}_2 \right) \Big\}$$

 $\{\text{DiagSet}[3, 6, 119],$ 
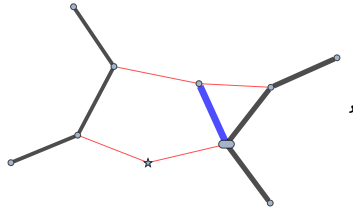
 $,$ 

$$\frac{G^3 m_1 m_2^2 \left( -4 \hat{n} \cdot \vec{a}_1 \hat{n} \times \vec{S}_1 \cdot \vec{v}_2 - 4 \hat{n} \cdot \vec{v}_1 \hat{n} \times \vec{S}_1 \cdot \vec{v}_2 \right)}{r^3} + \frac{1}{r^4} G^3 m_1 m_2^2 \left( 20 (\hat{n} \cdot \vec{v}_1)^2 \hat{n} \times \vec{S}_1 \cdot \vec{v}_2 + 4 \hat{n} \cdot \vec{v}_1 \vec{S}_1 \times \vec{v}_1 \cdot \vec{v}_2 - 12 \hat{n} \cdot \vec{v}_2 \hat{n} \cdot \vec{v}_1 \hat{n} \times \vec{S}_1 \cdot \vec{v}_2 - 4 (\hat{n} \cdot \vec{v}_2)^2 \hat{n} \times \vec{S}_1 \cdot \vec{v}_1 - 4 \vec{v}_1 \cdot \vec{v}_1 \hat{n} \times \vec{S}_1 \cdot \vec{v}_2 + 4 \vec{v}_1 \cdot \vec{v}_2 \hat{n} \times \vec{S}_1 \cdot \vec{v}_2 + 4 \vec{v}_2 \cdot \vec{v}_2 \hat{n} \times \vec{S}_1 \cdot \vec{v}_1 \right) \Big\}$$

 $\{\text{DiagSet}[3, 6, 120],$ 
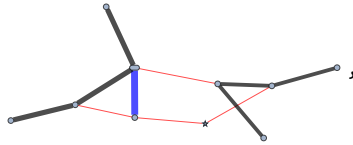

$$\frac{1}{r^3} G^3 m_1 m_2^2$$

$$\left( \frac{4}{3} \hat{n} \cdot \vec{a}_1 \hat{n} \times \vec{S}_1 \cdot \vec{v}_2 + \frac{4}{3} \hat{n} \cdot \vec{v}_2 \hat{n} \times \vec{S}_1 \cdot \vec{a}_1 - \frac{4}{3} \vec{S}_1 \times \vec{a}_1 \cdot \vec{v}_2 + \frac{4}{3} \hat{n} \cdot \vec{v}_1 \hat{n} \times \vec{S}_1 \cdot \vec{v}_2 + \frac{4}{3} \hat{n} \cdot \vec{v}_2 \hat{n} \times \vec{S}_1 \cdot \vec{v}_1 - \frac{4}{3} \vec{S}_1 \times \vec{v}_1 \cdot \vec{v}_2 \right) + \frac{1}{r^4} G^3 m_1 m_2^2 \left( -\frac{20}{3} (\hat{n} \cdot \vec{v}_1)^2 \hat{n} \times \vec{S}_1 \cdot \vec{v}_2 + \frac{8}{3} \hat{n} \cdot \vec{v}_1 \vec{S}_1 \times \vec{v}_1 \cdot \vec{v}_2 - \frac{20}{3} \hat{n} \cdot \vec{v}_2 \hat{n} \cdot \vec{v}_1 \hat{n} \times \vec{S}_1 \cdot \vec{v}_1 + \frac{4}{3} \hat{n} \cdot \vec{v}_2 \hat{n} \cdot \vec{v}_1 \hat{n} \times \vec{S}_1 \cdot \vec{v}_2 + \frac{4}{3} (\hat{n} \cdot \vec{v}_2)^2 \hat{n} \times \vec{S}_1 \cdot \vec{v}_1 - \frac{8}{3} \hat{n} \cdot \vec{v}_2 \vec{S}_1 \times \vec{v}_1 \cdot \vec{v}_2 + \frac{4}{3} \vec{v}_1 \cdot \vec{v}_1 \hat{n} \times \vec{S}_1 \cdot \vec{v}_2 + \frac{4}{3} \vec{v}_1 \cdot \vec{v}_2 \hat{n} \times \vec{S}_1 \cdot \vec{v}_1 + \frac{4}{3} \vec{v}_1 \cdot \vec{v}_2 \hat{n} \times \vec{S}_1 \cdot \vec{v}_2 + \frac{4}{3} \vec{v}_2 \cdot \vec{v}_2 \hat{n} \times \vec{S}_1 \cdot \vec{v}_1 \right) \Big\}$$

 $\{\text{DiagSet}[3, 6, 121],$ 
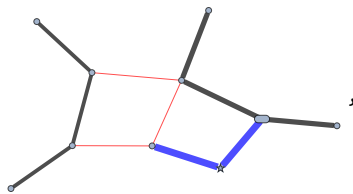
 $,$ 

$$\frac{1}{r^3} G^3 m_1 m_2^2 \left( \frac{7}{4} \hat{n} \cdot \vec{a}_1 \hat{n} \times \vec{S}_1 \cdot \vec{v}_1 + \frac{5}{4} \hat{n} \cdot \vec{v}_1 \hat{n} \times \vec{S}_1 \cdot \vec{a}_1 - \frac{3}{2} \hat{n} \cdot \vec{v}_2 \hat{n} \times \vec{S}_1 \cdot \vec{a}_1 + \frac{1}{2} \vec{S}_1 \times \vec{a}_1 \cdot \vec{v}_2 - \frac{1}{2} \vec{S}_1 \times \vec{v}_1 \cdot \vec{a}_1 + 3 \hat{n} \cdot \vec{v}_1 \hat{n} \times \vec{S}_1 \cdot \vec{v}_1 - \frac{3}{2} \hat{n} \cdot \vec{v}_2 \hat{n} \times \vec{S}_1 \cdot \vec{v}_1 + \frac{1}{2} \vec{S}_1 \times \vec{v}_1 \cdot \vec{v}_2 \right) + \frac{1}{r^4} G^3 m_1 m_2^2 \left( 5 (\hat{n} \cdot \vec{v}_1)^2 \hat{n} \times \vec{S}_1 \cdot \vec{v}_1 + \frac{3}{2} \hat{n} \cdot \vec{v}_1 \vec{S}_1 \times \vec{v}_1 \cdot \vec{v}_2 - \frac{15}{2} \hat{n} \cdot \vec{v}_2 \hat{n} \cdot \vec{v}_1 \hat{n} \times \vec{S}_1 \cdot \vec{v}_1 - \frac{1}{2} \vec{v}_1 \cdot \vec{v}_1 \hat{n} \times \vec{S}_1 \cdot \vec{v}_1 + \frac{3}{2} \vec{v}_1 \cdot \vec{v}_2 \hat{n} \times \vec{S}_1 \cdot \vec{v}_1 \right) \Big\}$$

{DiagSet[3, 6, 122],

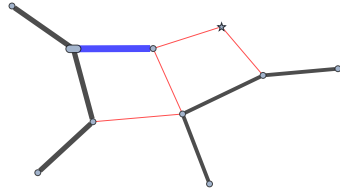

$$, \frac{1}{r^3} G^3 m_1 m_2^2$$

$$\left( \frac{1}{2} \hat{n} \cdot \vec{a}_1 \hat{n} \times \vec{S}_1 \cdot \vec{v}_2 + \frac{1}{2} \hat{n} \cdot \vec{v}_2 \hat{n} \times \vec{a}_1 \cdot \vec{S}_1 - \frac{1}{2} \vec{a}_1 \times \vec{S}_1 \cdot \vec{v}_2 + \frac{1}{2} \hat{n} \cdot \vec{v}_1 \hat{n} \times \vec{S}_1 \cdot \vec{v}_2 - \frac{1}{2} \hat{n} \cdot \vec{v}_2 \hat{n} \times \vec{S}_1 \cdot \vec{v}_1 + \frac{1}{2} \vec{S}_1 \times \vec{v}_1 \cdot \vec{v}_2 \right) +$$

$$\frac{1}{r^4} G^3 m_1 m_2^2 \left( -\frac{5}{2} (\hat{n} \cdot \vec{v}_1)^2 \hat{n} \times \vec{S}_1 \cdot \vec{v}_2 - 2 \hat{n} \cdot \vec{v}_1 \vec{S}_1 \times \vec{v}_1 \cdot \vec{v}_2 + \frac{5}{2} \hat{n} \cdot \vec{v}_2 \hat{n} \cdot \vec{v}_1 \hat{n} \times \vec{S}_1 \cdot \vec{v}_1 + \frac{5}{2} \hat{n} \cdot \vec{v}_2 \hat{n} \cdot \vec{v}_1 \hat{n} \times \vec{S}_1 \cdot \vec{v}_2 - \right.$$

$$\left. \frac{3}{2} (\hat{n} \cdot \vec{v}_2)^2 \hat{n} \times \vec{S}_1 \cdot \vec{v}_1 + \frac{3}{2} \hat{n} \cdot \vec{v}_2 \vec{S}_1 \times \vec{v}_1 \cdot \vec{v}_2 + \frac{1}{2} \vec{v}_1 \cdot \vec{v}_1 \hat{n} \times \vec{S}_1 \cdot \vec{v}_2 - \frac{1}{2} \vec{v}_1 \cdot \vec{v}_2 \hat{n} \times \vec{S}_1 \cdot \vec{v}_1 + \frac{1}{2} \vec{v}_2 \cdot \vec{v}_2 \hat{n} \times \vec{S}_1 \cdot \vec{v}_1 \right)$$

{DiagSet[3, 6, 123],

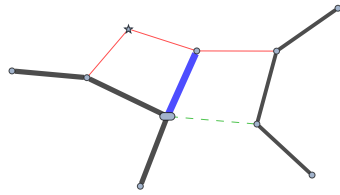

$$, \frac{1}{r^3} G^3 m_1 m_2^2$$

$$\left( -\frac{5}{3} \hat{n} \cdot \vec{a}_2 \hat{n} \times \vec{S}_1 \cdot \vec{v}_1 - \frac{5}{3} \hat{n} \cdot \vec{v}_1 \hat{n} \times \vec{S}_1 \cdot \vec{a}_2 + \frac{5}{3} \vec{S}_1 \times \vec{v}_1 \cdot \vec{a}_2 - \frac{5}{3} \hat{n} \cdot \vec{v}_1 \hat{n} \times \vec{S}_1 \cdot \vec{v}_2 - \frac{5}{3} \hat{n} \cdot \vec{v}_2 \hat{n} \times \vec{S}_1 \cdot \vec{v}_1 + \frac{5}{3} \vec{S}_1 \times \vec{v}_1 \cdot \vec{v}_2 \right) +$$

$$\frac{1}{r^4} G^3 m_1 m_2^2 \left( \frac{22}{3} (\hat{n} \cdot \vec{v}_1)^2 \hat{n} \times \vec{S}_1 \cdot \vec{v}_2 - \frac{7}{3} \hat{n} \cdot \vec{v}_1 \vec{S}_1 \times \vec{v}_1 \cdot \vec{v}_2 + \frac{16}{3} \hat{n} \cdot \vec{v}_2 \hat{n} \cdot \vec{v}_1 \hat{n} \times \vec{S}_1 \cdot \vec{v}_1 - \right.$$

$$\frac{25}{3} \hat{n} \cdot \vec{v}_2 \hat{n} \cdot \vec{v}_1 \hat{n} \times \vec{S}_1 \cdot \vec{v}_2 - \frac{25}{3} (\hat{n} \cdot \vec{v}_2)^2 \hat{n} \times \vec{S}_1 \cdot \vec{v}_1 + \frac{20}{3} \hat{n} \cdot \vec{v}_2 \vec{S}_1 \times \vec{v}_1 \cdot \vec{v}_2 -$$

$$\left. \frac{5}{3} \vec{v}_1 \cdot \vec{v}_1 \hat{n} \times \vec{S}_1 \cdot \vec{v}_2 + \frac{1}{3} \vec{v}_1 \cdot \vec{v}_2 \hat{n} \times \vec{S}_1 \cdot \vec{v}_1 + \frac{5}{3} \vec{v}_1 \cdot \vec{v}_2 \hat{n} \times \vec{S}_1 \cdot \vec{v}_2 + \frac{5}{3} \vec{v}_2 \cdot \vec{v}_2 \hat{n} \times \vec{S}_1 \cdot \vec{v}_1 \right)$$

{DiagSet[3, 6, 124],

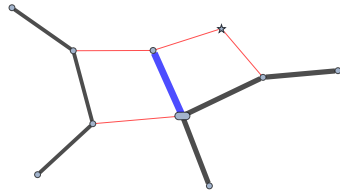

,

$$\frac{1}{r^3} G^3 m_1 m_2^2 \left( -\frac{5}{3} \hat{n} \cdot \vec{a}_1 \hat{n} \times \vec{S}_1 \cdot \vec{v}_1 + \frac{1}{3} \hat{n} \cdot \vec{v}_1 \hat{n} \times \vec{S}_1 \cdot \vec{a}_1 - \frac{5}{3} \vec{S}_1 \times \vec{v}_1 \cdot \vec{a}_1 - \frac{4}{3} \hat{n} \cdot \vec{v}_1 \hat{n} \times \vec{S}_1 \cdot \vec{v}_1 \right) + \frac{1}{r^4} G^3 m_1 m_2^2$$

$$\left( \frac{8}{3} (\hat{n} \cdot \vec{v}_1)^2 \hat{n} \times \vec{S}_1 \cdot \vec{v}_1 + \frac{4}{3} \hat{n} \cdot \vec{v}_1 \vec{S}_1 \times \vec{v}_1 \cdot \vec{v}_2 - \frac{20}{3} \hat{n} \cdot \vec{v}_2 \hat{n} \cdot \vec{v}_1 \hat{n} \times \vec{S}_1 \cdot \vec{v}_1 + \frac{8}{3} \vec{v}_1 \cdot \vec{v}_1 \hat{n} \times \vec{S}_1 \cdot \vec{v}_1 + \frac{4}{3} \vec{v}_1 \cdot \vec{v}_2 \hat{n} \times \vec{S}_1 \cdot \vec{v}_1 \right)$$

{DiagSet[3, 6, 125],

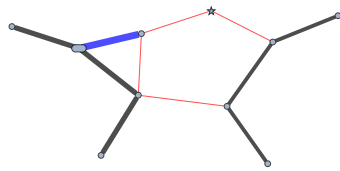

,

$$\frac{G^3 m_1 m_2^2 \left( \frac{1}{2} \hat{n} \cdot \vec{v}_2 \hat{n} \times \vec{S}_1 \cdot \vec{a}_1 - \frac{1}{4} \vec{S}_1 \times \vec{a}_1 \cdot \vec{v}_2 + \frac{1}{2} \hat{n} \cdot \vec{v}_2 \hat{n} \times \vec{S}_1 \cdot \vec{v}_1 - \frac{1}{4} \vec{S}_1 \times \vec{v}_1 \cdot \vec{v}_2 \right)}{r^3} + \frac{1}{r^4} G^3 m_1 m_2^2$$

$$\left( \frac{1}{2} (\hat{n} \cdot \vec{v}_2)^2 \hat{n} \times \vec{S}_1 \cdot \vec{v}_1 - \frac{1}{4} \hat{n} \cdot \vec{v}_2 \vec{S}_1 \times \vec{v}_1 \cdot \vec{v}_2 - \frac{5}{2} \hat{n} \cdot \vec{v}_1 \hat{n} \cdot \vec{v}_2 \hat{n} \times \vec{S}_1 \cdot \vec{v}_1 + \frac{3}{4} \hat{n} \cdot \vec{v}_1 \vec{S}_1 \times \vec{v}_1 \cdot \vec{v}_2 + \frac{1}{2} \vec{v}_1 \cdot \vec{v}_2 \hat{n} \times \vec{S}_1 \cdot \vec{v}_1 \right)$$

{DiagSet[3, 6, 126],

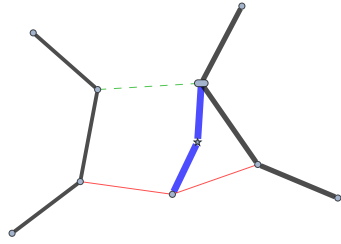

$$\frac{1}{r^3} G^3 m_1 m_2^2 \left( \hat{n} \cdot \vec{a}_2 \hat{n} \times \vec{S}_1 \cdot \vec{v}_1 - \frac{4}{3} \hat{n} \cdot \vec{a}_2 \hat{n} \times \vec{S}_1 \cdot \vec{v}_2 + \hat{n} \cdot \vec{v}_1 \hat{n} \times \vec{S}_1 \cdot \vec{a}_2 - \frac{4}{3} \hat{n} \cdot \vec{v}_2 \hat{n} \times \vec{S}_1 \cdot \vec{a}_2 - \vec{S}_1 \times \vec{v}_1 \cdot \vec{a}_2 + \frac{4}{3} \vec{S}_1 \times \vec{v}_2 \cdot \vec{a}_2 + \hat{n} \cdot \vec{v}_1 \hat{n} \times \vec{S}_1 \cdot \vec{v}_2 + \hat{n} \cdot \vec{v}_2 \hat{n} \times \vec{S}_1 \cdot \vec{v}_1 - \frac{8}{3} \hat{n} \cdot \vec{v}_2 \hat{n} \times \vec{S}_1 \cdot \vec{v}_2 - \left( \vec{S}_1 \times \vec{v}_1 \cdot \vec{v}_2 \right) \right) + \frac{1}{r^4} G^3 m_1 m_2^2 \left( -8 (\hat{n} \cdot \vec{v}_1)^2 \hat{n} \times \vec{S}_1 \cdot \vec{v}_2 - 3 \hat{n} \cdot \vec{v}_1 \vec{S}_1 \times \vec{v}_1 \cdot \vec{v}_2 + 2 \hat{n} \cdot \vec{v}_2 \hat{n} \cdot \vec{v}_1 \hat{n} \times \vec{S}_1 \cdot \vec{v}_1 + \frac{43}{3} \hat{n} \cdot \vec{v}_2 \hat{n} \cdot \vec{v}_1 \hat{n} \times \vec{S}_1 \cdot \vec{v}_2 + (\hat{n} \cdot \vec{v}_2)^2 \hat{n} \times \vec{S}_1 \cdot \vec{v}_1 - 8 (\hat{n} \cdot \vec{v}_2)^2 \hat{n} \times \vec{S}_1 \cdot \vec{v}_2 + \frac{2}{3} \hat{n} \cdot \vec{v}_2 \vec{S}_1 \times \vec{v}_1 \cdot \vec{v}_2 + \vec{v}_1 \cdot \vec{v}_1 \hat{n} \times \vec{S}_1 \cdot \vec{v}_2 - \vec{v}_1 \cdot \vec{v}_2 \hat{n} \times \vec{S}_1 \cdot \vec{v}_1 - \frac{5}{3} \vec{v}_1 \cdot \vec{v}_2 \hat{n} \times \vec{S}_1 \cdot \vec{v}_2 + \vec{v}_2 \cdot \vec{v}_2 \hat{n} \times \vec{S}_1 \cdot \vec{v}_1 \right) \Big\}$$

{DiagSet[3, 6, 127],

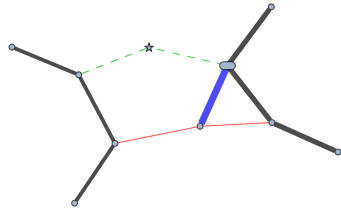

$$\frac{G^3 m_1 m_2^2 \left( 4 \hat{n} \cdot \vec{a}_2 \hat{n} \times \vec{S}_1 \cdot \vec{v}_2 - 4 \hat{n} \cdot \vec{v}_2 \hat{n} \times \vec{S}_1 \cdot \vec{a}_2 - 4 \vec{S}_1 \times \vec{v}_2 \cdot \vec{a}_2 \right)}{r^3} \Big\}$$

{DiagSet[3, 6, 128],

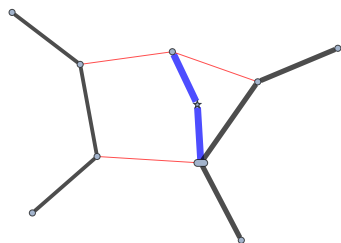

$$\frac{1}{r^3} G^3 m_1 m_2^2 \left( \hat{n} \cdot \vec{a}_1 \hat{n} \times \vec{S}_1 \cdot \vec{v}_1 - \frac{4}{3} \hat{n} \cdot \vec{a}_1 \hat{n} \times \vec{S}_1 \cdot \vec{v}_2 + 3 \hat{n} \cdot \vec{v}_1 \hat{n} \times \vec{S}_1 \cdot \vec{a}_1 - \frac{4}{3} \hat{n} \cdot \vec{v}_2 \hat{n} \times \vec{S}_1 \cdot \vec{a}_1 + \frac{4}{3} \vec{S}_1 \times \vec{a}_1 \cdot \vec{v}_2 + \vec{S}_1 \times \vec{v}_1 \cdot \vec{a}_1 + 4 \hat{n} \cdot \vec{v}_1 \hat{n} \times \vec{S}_1 \cdot \vec{v}_1 - \frac{4}{3} \hat{n} \cdot \vec{v}_1 \hat{n} \times \vec{S}_1 \cdot \vec{v}_2 - \frac{4}{3} \hat{n} \cdot \vec{v}_2 \hat{n} \times \vec{S}_1 \cdot \vec{v}_1 + \frac{4}{3} \vec{S}_1 \times \vec{v}_1 \cdot \vec{v}_2 \right) + \frac{1}{r^4} G^3 m_1 m_2^2 \left( -\frac{4}{3} (\hat{n} \cdot \vec{v}_1)^2 \hat{n} \times \vec{S}_1 \cdot \vec{v}_2 - \frac{2}{3} \hat{n} \cdot \vec{v}_1 \vec{S}_1 \times \vec{v}_1 \cdot \vec{v}_2 + \frac{8}{3} \hat{n} \cdot \vec{v}_2 \hat{n} \cdot \vec{v}_1 \hat{n} \times \vec{S}_1 \cdot \vec{v}_1 - \frac{4}{3} \hat{n} \cdot \vec{v}_2 \hat{n} \cdot \vec{v}_1 \hat{n} \times \vec{S}_1 \cdot \vec{v}_2 - \frac{4}{3} (\hat{n} \cdot \vec{v}_2)^2 \hat{n} \times \vec{S}_1 \cdot \vec{v}_1 + \frac{8}{3} \hat{n} \cdot \vec{v}_2 \vec{S}_1 \times \vec{v}_1 \cdot \vec{v}_2 + \frac{2}{3} \vec{v}_1 \cdot \vec{v}_1 \hat{n} \times \vec{S}_1 \cdot \vec{v}_2 + \frac{14}{3} \vec{v}_1 \cdot \vec{v}_2 \hat{n} \times \vec{S}_1 \cdot \vec{v}_1 - \frac{4}{3} \vec{v}_1 \cdot \vec{v}_2 \hat{n} \times \vec{S}_1 \cdot \vec{v}_2 - \frac{4}{3} \vec{v}_2 \cdot \vec{v}_2 \hat{n} \times \vec{S}_1 \cdot \vec{v}_1 \right) \Big\}$$

{DiagSet[3, 6, 129],

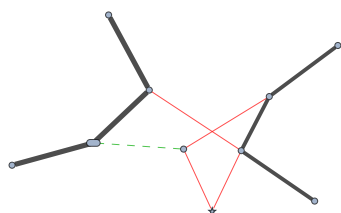



$$\frac{1}{r^3} G^3 m_1 m_2^2 \left( \frac{1}{2} \hat{n} \cdot \vec{a}_1 \hat{n} \times \vec{S}_1 \cdot \vec{v}_2 - \frac{3}{2} \hat{n} \cdot \vec{a}_2 \hat{n} \times \vec{S}_1 \cdot \vec{v}_2 + \frac{3}{2} \hat{n} \cdot \vec{v}_1 \hat{n} \times \vec{a}_2 \cdot \vec{S}_1 - \right. \\ \left. \frac{3}{2} \hat{n} \cdot \vec{v}_2 \hat{n} \times \vec{a}_2 \cdot \vec{S}_1 - \frac{1}{2} \vec{a}_2 \times \vec{S}_1 \cdot \vec{v}_1 + \vec{a}_2 \times \vec{S}_1 \cdot \vec{v}_2 - \frac{3}{2} \hat{n} \cdot \vec{v}_1 \hat{n} \times \vec{S}_1 \cdot \vec{v}_2 + \frac{3}{2} \hat{n} \cdot \vec{v}_2 \hat{n} \times \vec{S}_1 \cdot \vec{v}_2 \right) - \\ \frac{G^3 m_1 m_2^2 \hat{n} \times \vec{a}_2 \cdot \vec{S}_1}{2 r^2} + \frac{1}{r^4} G^3 m_1 m_2^2 \left( \frac{3}{2} (\hat{n} \cdot \vec{v}_1)^2 \hat{n} \times \vec{S}_1 \cdot \vec{v}_2 + \frac{3}{2} \hat{n} \cdot \vec{v}_1 \vec{S}_1 \times \vec{v}_1 \cdot \vec{v}_2 - \frac{5}{2} \hat{n} \cdot \vec{v}_2 \hat{n} \cdot \vec{v}_1 \hat{n} \times \vec{S}_1 \cdot \vec{v}_2 - \right. \\ \left. \frac{3}{2} \hat{n} \cdot \vec{v}_2 \vec{S}_1 \times \vec{v}_1 \cdot \vec{v}_2 + \frac{1}{2} \vec{v}_1 \cdot \vec{v}_1 \hat{n} \times \vec{S}_1 \cdot \vec{v}_2 - \vec{v}_1 \cdot \vec{v}_2 \hat{n} \times \vec{S}_1 \cdot \vec{v}_2 \right) \Big\}$$

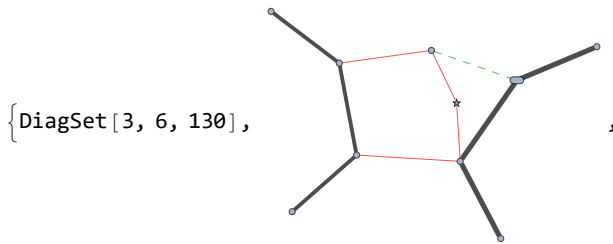

$$\frac{1}{r^3} G^3 m_1 m_2^2 \left( \frac{3}{4} \hat{n} \cdot \vec{a}_1 \hat{n} \times \vec{S}_1 \cdot \vec{v}_1 - \frac{3}{2} \hat{n} \cdot \vec{a}_2 \hat{n} \times \vec{S}_1 \cdot \vec{v}_1 - \frac{3}{4} \hat{n} \cdot \vec{v}_1 \hat{n} \times \vec{S}_1 \cdot \vec{a}_1 + \hat{n} \cdot \vec{v}_2 \hat{n} \times \vec{S}_1 \cdot \vec{a}_1 - \right. \\ \left. \frac{1}{2} \vec{S}_1 \times \vec{a}_1 \cdot \vec{v}_2 - \frac{1}{2} \vec{S}_1 \times \vec{v}_1 \cdot \vec{a}_1 + \frac{1}{2} \vec{S}_1 \times \vec{v}_1 \cdot \vec{a}_2 - \frac{3}{2} \hat{n} \cdot \vec{v}_1 \hat{n} \times \vec{S}_1 \cdot \vec{v}_1 + \frac{1}{2} \vec{S}_1 \times \vec{v}_1 \cdot \vec{v}_2 \right) + \\ \frac{G^3 m_1 m_2^2 \hat{n} \times \vec{S}_1 \cdot \vec{a}_1}{2 r^2} + \frac{1}{r^4} G^3 m_1 m_2^2 \left( -\frac{5}{2} (\hat{n} \cdot \vec{v}_2)^2 \hat{n} \times \vec{S}_1 \cdot \vec{v}_1 + \frac{1}{2} \hat{n} \cdot \vec{v}_2 \vec{S}_1 \times \vec{v}_1 \cdot \vec{v}_2 - \hat{n} \cdot \vec{v}_1 \hat{n} \cdot \vec{v}_2 \hat{n} \times \vec{S}_1 \cdot \vec{v}_1 + \right. \\ \left. \frac{3}{2} \hat{n} \cdot \vec{v}_1 \vec{S}_1 \times \vec{v}_1 \cdot \vec{v}_2 - \vec{v}_1 \cdot \vec{v}_2 \hat{n} \times \vec{S}_1 \cdot \vec{v}_1 + \frac{3}{2} \vec{v}_2 \cdot \vec{v}_2 \hat{n} \times \vec{S}_1 \cdot \vec{v}_1 \right) \Big\}$$

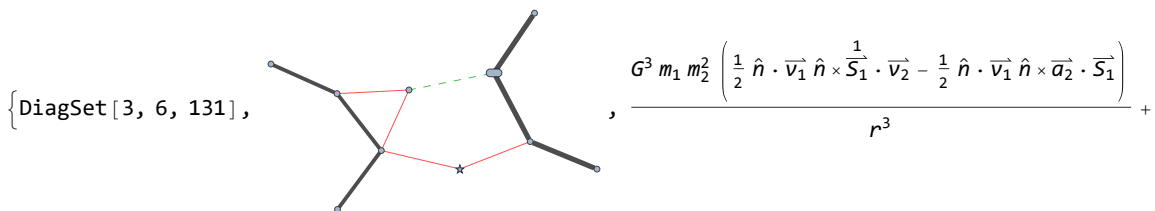

$$\frac{1}{r^4} G^3 m_1 m_2^2 \left( -2 (\hat{n} \cdot \vec{v}_1)^2 \hat{n} \times \vec{S}_1 \cdot \vec{v}_2 - \frac{1}{2} \hat{n} \cdot \vec{v}_1 \vec{S}_1 \times \vec{v}_1 \cdot \vec{v}_2 + \frac{5}{2} \hat{n} \cdot \vec{v}_2 \hat{n} \cdot \vec{v}_1 \hat{n} \times \vec{S}_1 \cdot \vec{v}_2 - \frac{1}{2} \vec{v}_1 \cdot \vec{v}_2 \hat{n} \times \vec{S}_1 \cdot \vec{v}_2 \right) \Big\}$$

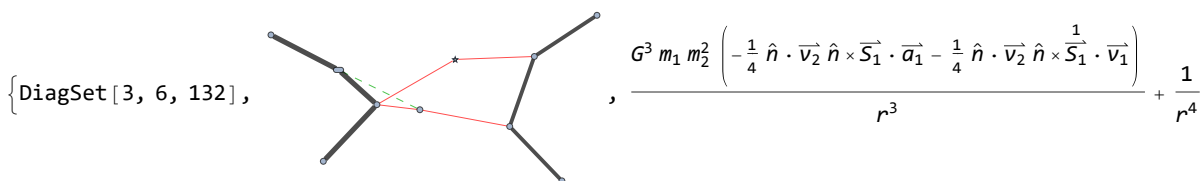

$$G^3 m_1 m_2^2 \left( (\hat{n} \cdot \vec{v}_2)^2 (-\hat{n} \times \vec{S}_1 \cdot \vec{v}_1) + \frac{1}{4} \hat{n} \cdot \vec{v}_2 \vec{S}_1 \times \vec{v}_1 \cdot \vec{v}_2 + \frac{5}{4} \hat{n} \cdot \vec{v}_1 \hat{n} \cdot \vec{v}_2 \hat{n} \times \vec{S}_1 \cdot \vec{v}_1 - \frac{1}{4} \vec{v}_1 \cdot \vec{v}_2 \hat{n} \times \vec{S}_1 \cdot \vec{v}_1 \right) \Big\}$$

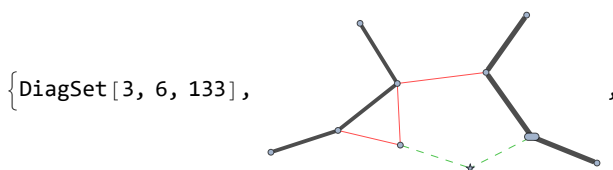

$$\frac{1}{r^3} G^3 m_1 m_2^2 \left( -\hat{n} \cdot \vec{v}_1 \hat{n} \times \vec{a}_2 \cdot \vec{S}_1 + \frac{1}{2} \vec{a}_2 \times \vec{S}_1 \cdot \vec{v}_1 + \frac{1}{2} \hat{n} \cdot \vec{v}_1 \hat{n} \times \vec{S}_1 \cdot \vec{v}_2 - \frac{3}{2} \hat{n} \cdot \vec{v}_2 \hat{n} \times \vec{S}_1 \cdot \vec{v}_2 \right) + \frac{G^3 m_1 m_2^2 \hat{n} \times \vec{a}_2 \cdot \vec{S}_1}{2 r^2} + \frac{1}{r^4} G^3 m_1 m_2^2$$

$$\left\{ \left( \hat{n} \cdot \vec{v}_1 \right)^2 \left( - \left( \hat{n} \times \vec{S}_1 \cdot \vec{v}_2 \right) \right) - \frac{1}{2} \hat{n} \cdot \vec{v}_1 \vec{S}_1 \times \vec{v}_1 \cdot \vec{v}_2 + 5 \hat{n} \cdot \vec{v}_2 \hat{n} \cdot \vec{v}_1 \hat{n} \times \vec{S}_1 \cdot \vec{v}_2 + \frac{3}{2} \hat{n} \cdot \vec{v}_2 \vec{S}_1 \times \vec{v}_1 \cdot \vec{v}_2 - \vec{v}_1 \cdot \vec{v}_2 \hat{n} \times \vec{S}_1 \cdot \vec{v}_2 \right\}$$

$\{ \text{DiagSet}[3, 6, 134],$

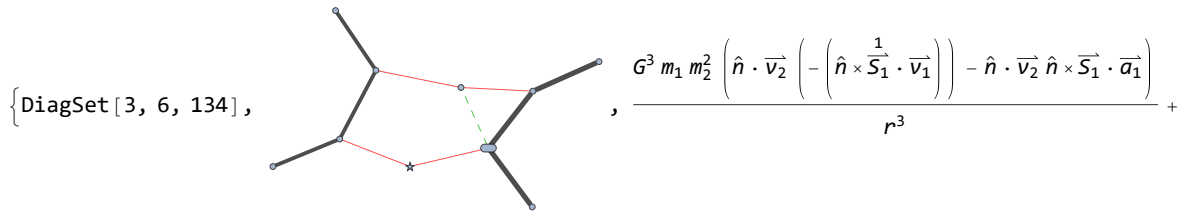

$, \frac{G^3 m_1 m_2^2 \left( \hat{n} \cdot \vec{v}_2 \left( - \left( \hat{n} \times \vec{S}_1 \cdot \vec{v}_1 \right) \right) - \hat{n} \cdot \vec{v}_2 \hat{n} \times \vec{S}_1 \cdot \vec{a}_1 \right)}{r^3} +$

$$\frac{1}{r^4} G^3 m_1 m_2^2 \left( -4 \left( \hat{n} \cdot \vec{v}_2 \right)^2 \hat{n} \times \vec{S}_1 \cdot \vec{v}_1 + \hat{n} \cdot \vec{v}_2 \vec{S}_1 \times \vec{v}_1 \cdot \vec{v}_2 + 5 \hat{n} \cdot \vec{v}_1 \hat{n} \cdot \vec{v}_2 \hat{n} \times \vec{S}_1 \cdot \vec{v}_1 - \vec{v}_1 \cdot \vec{v}_2 \hat{n} \times \vec{S}_1 \cdot \vec{v}_1 \right) \}$$

$\{ \text{DiagSet}[3, 6, 135],$

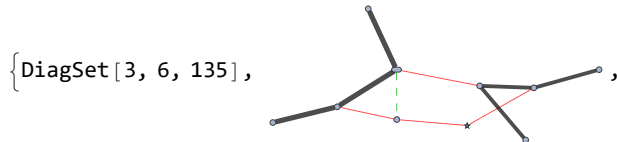

$,$

$$\frac{G^3 m_1 m_2^2 \left( -2 \hat{n} \cdot \vec{v}_2 \hat{n} \times \vec{S}_1 \cdot \vec{a}_1 + \vec{S}_1 \times \vec{a}_1 \cdot \vec{v}_2 - 2 \hat{n} \cdot \vec{v}_2 \hat{n} \times \vec{S}_1 \cdot \vec{v}_1 + \frac{1}{\vec{S}_1 \times \vec{v}_1 \cdot \vec{v}_2} \right)}{r^3} + \frac{1}{r^4}$$

$$G^3 m_1 m_2^2 \left( -2 \left( \hat{n} \cdot \vec{v}_2 \right)^2 \hat{n} \times \vec{S}_1 \cdot \vec{v}_1 + \hat{n} \cdot \vec{v}_2 \vec{S}_1 \times \vec{v}_1 \cdot \vec{v}_2 + 10 \hat{n} \cdot \vec{v}_1 \hat{n} \cdot \vec{v}_2 \hat{n} \times \vec{S}_1 \cdot \vec{v}_1 - 3 \hat{n} \cdot \vec{v}_1 \vec{S}_1 \times \vec{v}_1 \cdot \vec{v}_2 - 2 \vec{v}_1 \cdot \vec{v}_2 \hat{n} \times \vec{S}_1 \cdot \vec{v}_1 \right) \}$$

$\{ \text{DiagSet}[3, 6, 136],$

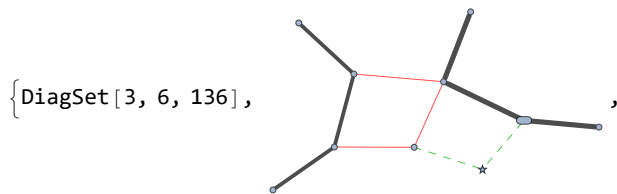

$,$

$$\frac{1}{r^3} G^3 m_1 m_2^2 \left( \frac{5}{4} \hat{n} \cdot \vec{a}_1 \hat{n} \times \vec{S}_1 \cdot \vec{v}_1 + \frac{1}{2} \hat{n} \cdot \vec{a}_2 \hat{n} \times \vec{S}_1 \cdot \vec{v}_1 - \frac{1}{4} \hat{n} \cdot \vec{v}_1 \hat{n} \times \vec{S}_1 \cdot \vec{a}_1 - \right.$$

$$\left. \frac{1}{2} \vec{S}_1 \times \vec{v}_1 \cdot \vec{a}_1 - \frac{1}{2} \vec{S}_1 \times \vec{v}_1 \cdot \vec{a}_2 - \frac{5}{2} \hat{n} \cdot \vec{v}_1 \hat{n} \times \vec{S}_1 \cdot \vec{v}_1 + \hat{n} \cdot \vec{v}_2 \hat{n} \times \vec{S}_1 \cdot \vec{v}_1 \right) + \frac{G^3 m_1 m_2^2 \hat{n} \times \vec{S}_1 \cdot \vec{a}_1}{2 r^2} +$$

$$\frac{1}{r^4} G^3 m_1 m_2^2 \left( -4 \left( \hat{n} \cdot \vec{v}_1 \right)^2 \hat{n} \times \vec{S}_1 \cdot \vec{v}_1 + 4 \hat{n} \cdot \vec{v}_2 \hat{n} \cdot \vec{v}_1 \hat{n} \times \vec{S}_1 \cdot \vec{v}_1 + \frac{5}{2} \left( \hat{n} \cdot \vec{v}_2 \right)^2 \hat{n} \times \vec{S}_1 \cdot \vec{v}_1 - \right.$$

$$\left. 2 \hat{n} \cdot \vec{v}_2 \vec{S}_1 \times \vec{v}_1 \cdot \vec{v}_2 + \frac{1}{2} \vec{v}_1 \cdot \vec{v}_1 \hat{n} \times \vec{S}_1 \cdot \vec{v}_1 - \vec{v}_1 \cdot \vec{v}_2 \hat{n} \times \vec{S}_1 \cdot \vec{v}_1 - \frac{1}{2} \vec{v}_2 \cdot \vec{v}_2 \hat{n} \times \vec{S}_1 \cdot \vec{v}_1 \right) \}$$

$\{ \text{DiagSet}[3, 6, 137],$

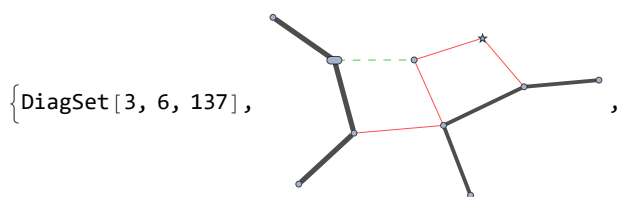

$,$

$$\frac{1}{r^3} G^3 m_1 m_2^2 \left( \frac{1}{2} \hat{n} \cdot \vec{a}_1 \hat{n} \times \vec{S}_1 \cdot \vec{v}_2 - \frac{3}{2} \hat{n} \cdot \vec{a}_2 \hat{n} \times \vec{S}_1 \cdot \vec{v}_2 + \frac{3}{2} \hat{n} \cdot \vec{v}_1 \hat{n} \times \vec{a}_2 \cdot \vec{S}_1 - \right.$$

$$\left. \frac{3}{2} \hat{n} \cdot \vec{v}_2 \hat{n} \times \vec{a}_2 \cdot \vec{S}_1 - \frac{1}{2} \vec{a}_2 \times \vec{S}_1 \cdot \vec{v}_1 + \vec{a}_2 \times \vec{S}_1 \cdot \vec{v}_2 + \frac{1}{2} \hat{n} \cdot \vec{v}_1 \hat{n} \times \vec{S}_1 \cdot \vec{v}_2 - \frac{1}{2} \hat{n} \cdot \vec{v}_2 \hat{n} \times \vec{S}_1 \cdot \vec{v}_2 \right) -$$

$$\frac{G^3 m_1 m_2^2 \hat{n} \times \vec{a}_2 \cdot \vec{S}_1}{2 r^2} + \frac{1}{r^4} G^3 m_1 m_2^2 \left( -\frac{5}{2} \left( \hat{n} \cdot \vec{v}_1 \right)^2 \hat{n} \times \vec{S}_1 \cdot \vec{v}_2 - \frac{1}{2} \hat{n} \cdot \vec{v}_1 \vec{S}_1 \times \vec{v}_1 \cdot \vec{v}_2 + \frac{9}{2} \hat{n} \cdot \vec{v}_2 \hat{n} \cdot \vec{v}_1 \hat{n} \times \vec{S}_1 \cdot \vec{v}_2 - \right.$$

$$\left. 3 \left( \hat{n} \cdot \vec{v}_2 \right)^2 \hat{n} \times \vec{S}_1 \cdot \vec{v}_2 + \frac{1}{2} \hat{n} \cdot \vec{v}_2 \vec{S}_1 \times \vec{v}_1 \cdot \vec{v}_2 + \frac{1}{2} \vec{v}_1 \cdot \vec{v}_1 \hat{n} \times \vec{S}_1 \cdot \vec{v}_2 - \vec{v}_1 \cdot \vec{v}_2 \hat{n} \times \vec{S}_1 \cdot \vec{v}_2 \right) \}$$

{DiagSet[3, 6, 138],

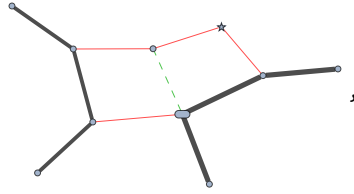

$$\frac{1}{r^3} G^3 m_1 m_2^2 \left( \hat{n} \cdot \vec{a}_1 \hat{n} \times \vec{S}_1 \cdot \vec{v}_1 - 4 \hat{n} \cdot \vec{a}_2 \hat{n} \times \vec{S}_1 \cdot \vec{v}_1 - 5 \hat{n} \cdot \vec{v}_1 \hat{n} \times \vec{S}_1 \cdot \vec{a}_1 + 6 \hat{n} \cdot \vec{v}_2 \hat{n} \times \vec{S}_1 \cdot \vec{a}_1 - \right. \\ \left. 2 \vec{S}_1 \times \vec{a}_1 \cdot \vec{v}_2 - 2 \vec{S}_1 \times \vec{v}_1 \cdot \vec{a}_1 + 2 \vec{S}_1 \times \vec{v}_1 \cdot \vec{a}_2 - 2 \hat{n} \cdot \vec{v}_1 \hat{n} \times \vec{S}_1 \cdot \vec{v}_1 - 4 \hat{n} \cdot \vec{v}_2 \hat{n} \times \vec{S}_1 \cdot \vec{v}_1 + 2 \vec{S}_1 \times \vec{v}_1 \cdot \vec{v}_2 \right) + \\ \frac{2 G^3 m_1 m_2^2 \hat{n} \times \vec{S}_1 \cdot \vec{a}_1}{r^2} + \frac{1}{r^4} G^3 m_1 m_2^2 \left( 4 (\hat{n} \cdot \vec{v}_1)^2 \hat{n} \times \vec{S}_1 \cdot \vec{v}_1 - 2 \hat{n} \cdot \vec{v}_1 \vec{S}_1 \times \vec{v}_1 \cdot \vec{v}_2 + 2 \hat{n} \cdot \vec{v}_2 \hat{n} \cdot \vec{v}_1 \hat{n} \times \vec{S}_1 \cdot \vec{v}_1 - \right. \\ \left. 20 (\hat{n} \cdot \vec{v}_2)^2 \hat{n} \times \vec{S}_1 \cdot \vec{v}_1 + 10 \hat{n} \cdot \vec{v}_2 \vec{S}_1 \times \vec{v}_1 \cdot \vec{v}_2 - 2 \vec{v}_1 \cdot \vec{v}_1 \hat{n} \times \vec{S}_1 \cdot \vec{v}_1 + 4 \vec{v}_2 \cdot \vec{v}_2 \hat{n} \times \vec{S}_1 \cdot \vec{v}_1 \right) \}$$

{DiagSet[3, 6, 139],

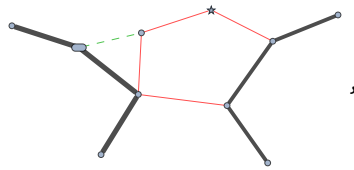

$$\frac{G^3 m_1 m_2^2 \left( -\frac{1}{2} \hat{n} \cdot \vec{v}_2 \hat{n} \times \vec{S}_1 \cdot \vec{a}_1 + \frac{1}{4} \vec{S}_1 \times \vec{a}_1 \cdot \vec{v}_2 - \frac{1}{2} \hat{n} \cdot \vec{v}_2 \hat{n} \times \vec{S}_1 \cdot \vec{v}_1 + \frac{1}{4} \vec{S}_1 \times \vec{v}_1 \cdot \vec{v}_2 \right)}{r^3} + \frac{1}{r^4} G^3 m_1 m_2^2 \\ \left( -\frac{1}{2} (\hat{n} \cdot \vec{v}_2)^2 \hat{n} \times \vec{S}_1 \cdot \vec{v}_1 + \frac{1}{4} \hat{n} \cdot \vec{v}_2 \vec{S}_1 \times \vec{v}_1 \cdot \vec{v}_2 + \frac{5}{2} \hat{n} \cdot \vec{v}_1 \hat{n} \cdot \vec{v}_2 \hat{n} \times \vec{S}_1 \cdot \vec{v}_1 - \frac{3}{4} \hat{n} \cdot \vec{v}_1 \vec{S}_1 \times \vec{v}_1 \cdot \vec{v}_2 - \frac{1}{2} \vec{v}_1 \cdot \vec{v}_2 \hat{n} \times \vec{S}_1 \cdot \vec{v}_1 \right) \}$$

{DiagSet[3, 6, 140],

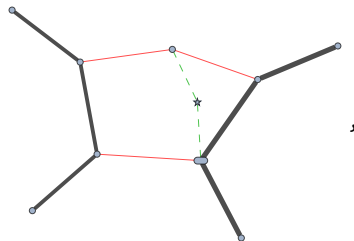

$$\frac{1}{r^3} G^3 m_1 m_2^2 \left( 3 \hat{n} \cdot \vec{a}_1 \hat{n} \times \vec{S}_1 \cdot \vec{v}_1 + 4 \hat{n} \cdot \vec{a}_2 \hat{n} \times \vec{S}_1 \cdot \vec{v}_1 - 3 \hat{n} \cdot \vec{v}_1 \hat{n} \times \vec{S}_1 \cdot \vec{a}_1 + \right. \\ \left. 2 \hat{n} \cdot \vec{v}_2 \hat{n} \times \vec{S}_1 \cdot \vec{a}_1 - 2 \vec{S}_1 \times \vec{v}_1 \cdot \vec{a}_1 - 2 \vec{S}_1 \times \vec{v}_1 \cdot \vec{a}_2 - 6 \hat{n} \cdot \vec{v}_1 \hat{n} \times \vec{S}_1 \cdot \vec{v}_1 \right) + \frac{2 G^3 m_1 m_2^2 \hat{n} \times \vec{S}_1 \cdot \vec{a}_1}{r^2} + \frac{1}{r^4} \\ G^3 m_1 m_2^2 \left( 16 (\hat{n} \cdot \vec{v}_2)^2 \hat{n} \times \vec{S}_1 \cdot \vec{v}_1 - 8 \hat{n} \cdot \vec{v}_2 \vec{S}_1 \times \vec{v}_1 \cdot \vec{v}_2 - 6 \hat{n} \cdot \vec{v}_1 \hat{n} \cdot \vec{v}_2 \hat{n} \times \vec{S}_1 \cdot \vec{v}_1 - 4 \vec{v}_2 \cdot \vec{v}_2 \hat{n} \times \vec{S}_1 \cdot \vec{v}_1 \right) \}$$

{DiagSet[3, 7, 1],

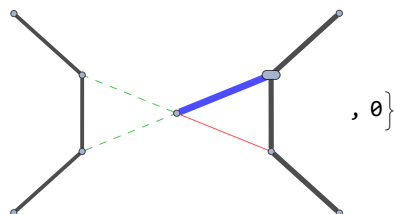

, 0}

$$\begin{aligned}
& \left\{ \text{DiagSet}[3, 7, 2], \right. \\
& \quad \left. , \emptyset \right\} \\
& \left\{ \text{DiagSet}[3, 7, 3], \right. \\
& \quad \left. , \frac{\pi^2 G^3 m_1 m_2^2 \left( \frac{9}{2} \vec{v}_2 \cdot \vec{v}_2 \hat{n} \times \vec{S}_1 \cdot \vec{v}_2 - \frac{45}{2} (\hat{n} \cdot \vec{v}_2)^2 \hat{n} \times \vec{S}_1 \cdot \vec{v}_2 \right)}{r^4} \right\} \\
& \left\{ \text{DiagSet}[3, 7, 4], \right. \\
& \quad \left. , \frac{\pi^2 G^3 m_1 m_2^2 \left( -\frac{45}{2} (\hat{n} \cdot \vec{v}_1)^2 \hat{n} \times \vec{S}_1 \cdot \vec{v}_2 - 9 \hat{n} \cdot \vec{v}_1 \vec{S}_1 \times \vec{v}_1 \cdot \vec{v}_2 + \frac{9}{2} \vec{v}_1 \cdot \vec{v}_1 \hat{n} \times \vec{S}_1 \cdot \vec{v}_2 \right)}{r^4} \right\} \\
& \left\{ \text{DiagSet}[3, 7, 5], \right. \\
& \quad \left. , \frac{\pi^2 G^3 m_1 m_2^2 \left( \frac{15}{2} (\hat{n} \cdot \vec{v}_2)^2 \hat{n} \times \vec{S}_1 \cdot \vec{v}_1 - 3 \hat{n} \cdot \vec{v}_2 \vec{S}_1 \times \vec{v}_1 \cdot \vec{v}_2 - \frac{3}{2} \vec{v}_2 \cdot \vec{v}_2 \hat{n} \times \vec{S}_1 \cdot \vec{v}_1 \right)}{r^4} \right\} \\
& \left\{ \text{DiagSet}[3, 7, 6], \right. \\
& \quad \left. , \frac{\frac{1}{r^3} \pi^2 G^3 m_1 m_2^2 \left( -3 \hat{n} \cdot \vec{a}_2 \hat{n} \times \vec{S}_1 \cdot \vec{v}_2 + 3 \hat{n} \cdot \vec{v}_2 \hat{n} \times \vec{S}_1 \cdot \vec{a}_2 + 2 \vec{S}_1 \times \vec{v}_2 \cdot \vec{a}_2 - 12 \hat{n} \cdot \vec{v}_2 \hat{n} \times \vec{S}_1 \cdot \vec{v}_2 \right) + \pi^2 G^3 m_1 m_2^2 \left( 9 \hat{n} \cdot \vec{v}_2 \vec{S}_1 \times \vec{v}_1 \cdot \vec{v}_2 + 45 \hat{n} \cdot \vec{v}_1 \hat{n} \cdot \vec{v}_2 \hat{n} \times \vec{S}_1 \cdot \vec{v}_2 - 9 \vec{v}_1 \cdot \vec{v}_2 \hat{n} \times \vec{S}_1 \cdot \vec{v}_2 \right)}{r^4} \right\} \\
& \left\{ \text{DiagSet}[3, 7, 7], \right. \\
& \quad \left. , \right\}
\end{aligned}$$

$$\frac{1}{r^3} \pi^2 G^3 m_1 m_2^2 \left( -3 \hat{n} \cdot \vec{a}_1 \hat{n} \times \vec{S}_1 \cdot \vec{v}_2 - 12 \hat{n} \cdot \vec{a}_2 \hat{n} \times \vec{S}_1 \cdot \vec{v}_1 + 12 \hat{n} \cdot \vec{v}_1 \hat{n} \times \vec{S}_1 \cdot \vec{a}_2 + \right. \\ \left. 3 \hat{n} \cdot \vec{v}_2 \hat{n} \times \vec{S}_1 \cdot \vec{a}_1 - 2 \vec{S}_1 \times \vec{a}_1 \cdot \vec{v}_2 + 8 \vec{S}_1 \times \vec{v}_1 \cdot \vec{a}_2 - 3 \hat{n} \cdot \vec{v}_1 \hat{n} \times \vec{S}_1 \cdot \vec{v}_2 - 3 \hat{n} \cdot \vec{v}_2 \hat{n} \times \vec{S}_1 \cdot \vec{v}_1 \right) + \\ \frac{1}{r^4} \pi^2 G^3 m_1 m_2^2 \left( 15 (\hat{n} \cdot \vec{v}_1)^2 \hat{n} \times \vec{S}_1 \cdot \vec{v}_2 + 3 \hat{n} \cdot \vec{v}_1 \vec{S}_1 \times \vec{v}_1 \cdot \vec{v}_2 + 15 \hat{n} \cdot \vec{v}_2 \hat{n} \cdot \vec{v}_1 \hat{n} \times \vec{S}_1 \cdot \vec{v}_1 + \right. \\ \left. 30 \hat{n} \cdot \vec{v}_2 \hat{n} \cdot \vec{v}_1 \hat{n} \times \vec{S}_1 \cdot \vec{v}_2 - 30 (\hat{n} \cdot \vec{v}_2)^2 \hat{n} \times \vec{S}_1 \cdot \vec{v}_1 + 18 \hat{n} \cdot \vec{v}_2 \vec{S}_1 \times \vec{v}_1 \cdot \vec{v}_2 - \right. \\ \left. 3 \vec{v}_1 \cdot \vec{v}_1 \hat{n} \times \vec{S}_1 \cdot \vec{v}_2 - 3 \vec{v}_1 \cdot \vec{v}_2 \hat{n} \times \vec{S}_1 \cdot \vec{v}_1 - 6 \vec{v}_1 \cdot \vec{v}_2 \hat{n} \times \vec{S}_1 \cdot \vec{v}_2 + 6 \vec{v}_2 \cdot \vec{v}_2 \hat{n} \times \vec{S}_1 \cdot \vec{v}_1 \right) \Big\}$$

{DiagSet[3, 7, 8], 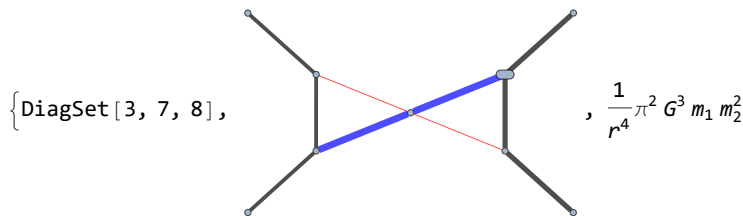 ,  $\frac{1}{r^4} \pi^2 G^3 m_1 m_2^2$

$$\left( -\frac{15}{4} (\hat{n} \cdot \vec{v}_2)^2 \hat{n} \times \vec{S}_1 \cdot \vec{v}_1 + \frac{9}{4} \hat{n} \cdot \vec{v}_2 \vec{S}_1 \times \vec{v}_1 \cdot \vec{v}_2 + \frac{15}{4} \hat{n} \cdot \vec{v}_1 \hat{n} \cdot \vec{v}_2 \hat{n} \times \vec{S}_1 \cdot \vec{v}_2 - \frac{3}{4} \vec{v}_1 \cdot \vec{v}_2 \hat{n} \times \vec{S}_1 \cdot \vec{v}_2 + \frac{3}{4} \vec{v}_2 \cdot \vec{v}_2 \hat{n} \times \vec{S}_1 \cdot \vec{v}_1 \right) \Big\}$$

{DiagSet[3, 7, 9], 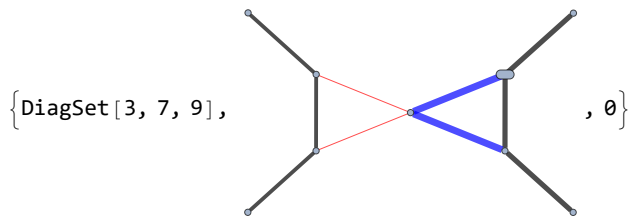 , 0}

{DiagSet[3, 7, 10], 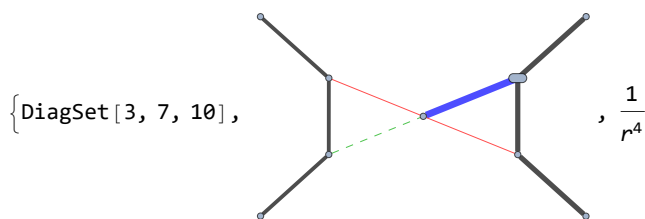 ,  $\frac{1}{r^4}$

$$\pi^2 G^3 m_1 m_2^2 \left( -\frac{15}{8} (\hat{n} \cdot \vec{v}_1)^2 \hat{n} \times \vec{S}_1 \cdot \vec{v}_2 - \frac{3}{4} \hat{n} \cdot \vec{v}_1 \vec{S}_1 \times \vec{v}_1 \cdot \vec{v}_2 - \frac{15}{8} \hat{n} \cdot \vec{v}_2 \hat{n} \cdot \vec{v}_1 \hat{n} \times \vec{S}_1 \cdot \vec{v}_2 - \right. \\ \left. \frac{3}{8} \hat{n} \cdot \vec{v}_2 \vec{S}_1 \times \vec{v}_1 \cdot \vec{v}_2 + \frac{3}{8} \vec{v}_1 \cdot \vec{v}_1 \hat{n} \times \vec{S}_1 \cdot \vec{v}_2 + \frac{3}{8} \vec{v}_1 \cdot \vec{v}_2 \hat{n} \times \vec{S}_1 \cdot \vec{v}_2 \right) \Big\}$$

{DiagSet[3, 7, 11], 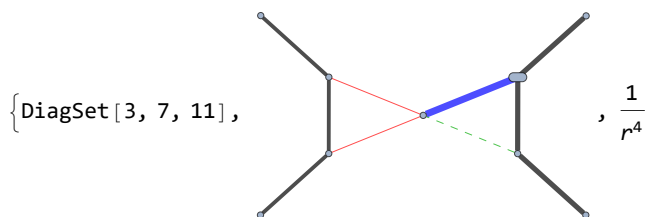 ,  $\frac{1}{r^4}$

$$\pi^2 G^3 m_1 m_2^2 \left( -\frac{3}{8} \hat{n} \cdot \vec{v}_1 \vec{S}_1 \times \vec{v}_1 \cdot \vec{v}_2 + \frac{15}{8} \hat{n} \cdot \vec{v}_2 \hat{n} \cdot \vec{v}_1 \hat{n} \times \vec{S}_1 \cdot \vec{v}_1 - \frac{3}{8} \vec{v}_1 \cdot \vec{v}_2 \hat{n} \times \vec{S}_1 \cdot \vec{v}_1 \right) \Big\}$$

{DiagSet[3, 7, 12], 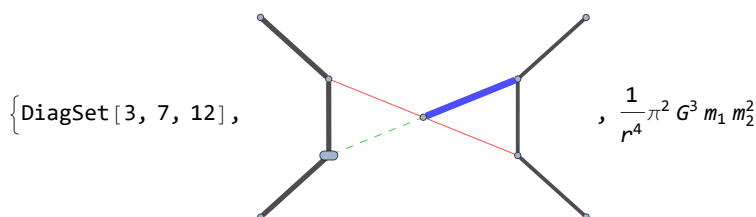 ,  $\frac{1}{r^4} \pi^2 G^3 m_1 m_2^2$

$$\left\{ -\frac{15}{8} (\hat{n} \cdot \vec{v}_2)^2 \hat{n} \times \vec{S}_1 \cdot \vec{v}_2 - \frac{3}{8} \hat{n} \cdot \vec{v}_2 \vec{S}_1 \times \vec{v}_1 \cdot \vec{v}_2 - \frac{15}{8} \hat{n} \cdot \vec{v}_1 \hat{n} \cdot \vec{v}_2 \hat{n} \times \vec{S}_1 \cdot \vec{v}_2 + \frac{3}{8} \vec{v}_1 \cdot \vec{v}_2 \hat{n} \times \vec{S}_1 \cdot \vec{v}_2 + \frac{3}{8} \vec{v}_2 \cdot \vec{v}_2 \hat{n} \times \vec{S}_1 \cdot \vec{v}_2 \right\}$$

$$\left\{ \text{DiagSet}[3, 7, 13], \frac{1}{r^4} \right\}$$
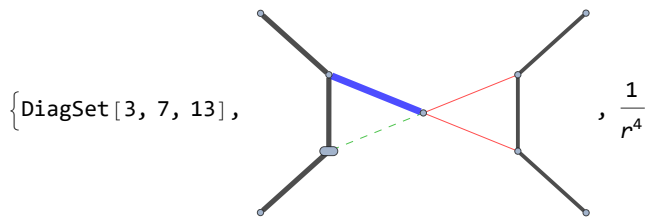

$$\pi^2 G^3 m_1 m_2^2 \left\{ -\frac{3}{8} \hat{n} \cdot \vec{v}_1 \vec{S}_1 \times \vec{v}_1 \cdot \vec{v}_2 + \frac{15}{8} \hat{n} \cdot \vec{v}_2 \hat{n} \cdot \vec{v}_1 \hat{n} \times \vec{S}_1 \cdot \vec{v}_1 - \frac{3}{8} \vec{v}_1 \cdot \vec{v}_2 \hat{n} \times \vec{S}_1 \cdot \vec{v}_1 \right\}$$

$$\left\{ \text{DiagSet}[3, 7, 14], \right\}$$
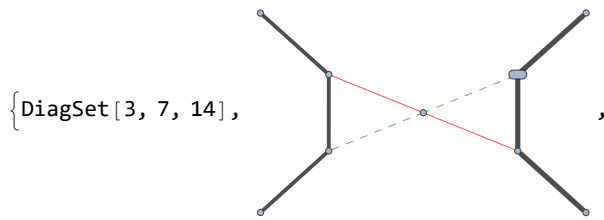

$$\frac{\pi^2 G^3 m_1 m_2^2 \left\{ \frac{3}{4} \hat{n} \cdot \vec{v}_2 \vec{S}_1 \times \vec{v}_1 \cdot \vec{v}_2 + \frac{15}{4} \hat{n} \cdot \vec{v}_1 \hat{n} \cdot \vec{v}_2 \hat{n} \times \vec{S}_1 \cdot \vec{v}_2 - \frac{3}{4} \vec{v}_1 \cdot \vec{v}_2 \hat{n} \times \vec{S}_1 \cdot \vec{v}_2 \right\}}{r^4}$$

$$\left\{ \text{DiagSet}[3, 7, 15], \right\}$$
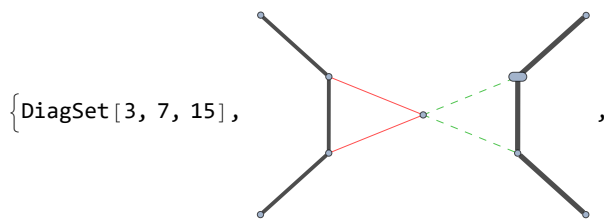

$$\frac{\pi^2 G^3 m_1 m_2^2 \left\{ -\frac{15}{8} (\hat{n} \cdot \vec{v}_2)^2 \hat{n} \times \vec{S}_1 \cdot \vec{v}_1 + \frac{3}{4} \hat{n} \cdot \vec{v}_2 \vec{S}_1 \times \vec{v}_1 \cdot \vec{v}_2 + \frac{3}{8} \vec{v}_2 \cdot \vec{v}_2 \hat{n} \times \vec{S}_1 \cdot \vec{v}_1 \right\}}{r^4}$$

$$\left\{ \text{DiagSet}[3, 7, 16], \emptyset \right\}$$
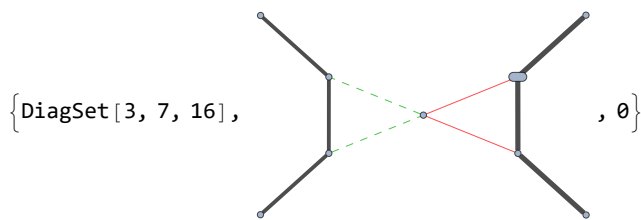

$$\left\{ \text{DiagSet}[3, 7, 17], \emptyset \right\}$$
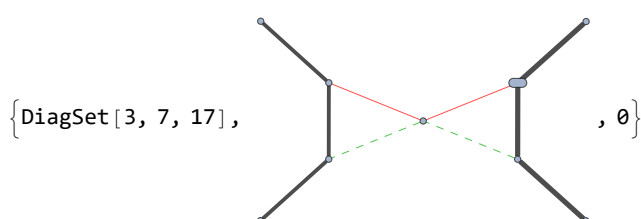

$$\left\{ \text{DiagSet}[3, 7, 18], \frac{1}{r^4} \right\}$$
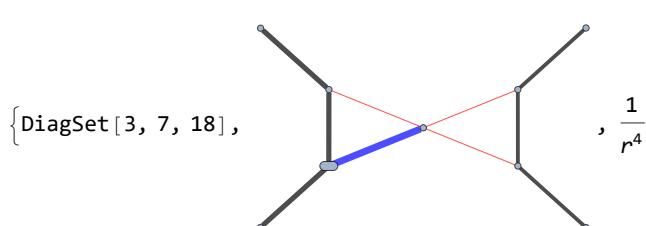

$$\pi^2 G^3 m_1 m_2^2 \left( -\frac{15}{8} (\hat{n} \cdot \vec{v}_2)^2 \hat{n} \times \vec{S}_1 \cdot \vec{v}_1 + \frac{3}{4} \hat{n} \cdot \vec{v}_2 \vec{S}_1 \times \vec{v}_1 \cdot \vec{v}_2 + \frac{15}{4} \hat{n} \cdot \vec{v}_1 \hat{n} \cdot \vec{v}_2 \hat{n} \times \vec{S}_1 \cdot \vec{v}_1 - \right. \\ \left. \frac{3}{4} \hat{n} \cdot \vec{v}_1 \vec{S}_1 \times \vec{v}_1 \cdot \vec{v}_2 - \frac{3}{4} \vec{v}_1 \cdot \vec{v}_2 \hat{n} \times \vec{S}_1 \cdot \vec{v}_1 + \frac{3}{8} \vec{v}_2 \cdot \vec{v}_2 \hat{n} \times \vec{S}_1 \cdot \vec{v}_1 \right) \}$$

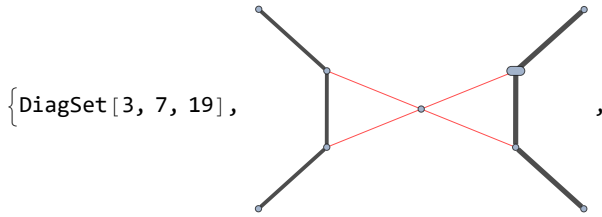

$$\frac{1}{r^3} \pi^2 G^3 m_1 m_2^2 \left( -\frac{3}{2} \hat{n} \cdot \vec{v}_1 \hat{n} \times \vec{S}_1 \cdot \vec{a}_1 + 6 \hat{n} \cdot \vec{v}_2 \hat{n} \times \vec{S}_1 \cdot \vec{a}_1 - 2 \vec{S}_1 \times \vec{a}_1 \cdot \vec{v}_2 - \right. \\ \left. \frac{1}{2} \vec{S}_1 \times \vec{v}_1 \cdot \vec{a}_1 - \frac{3}{2} \hat{n} \cdot \vec{v}_1 \hat{n} \times \vec{S}_1 \cdot \vec{v}_1 + 6 \hat{n} \cdot \vec{v}_2 \hat{n} \times \vec{S}_1 \cdot \vec{v}_1 - 2 \vec{S}_1 \times \vec{v}_1 \cdot \vec{v}_2 \right) + \frac{1}{r^4} \\ \pi^2 G^3 m_1 m_2^2 \left( \frac{15}{4} (\hat{n} \cdot \vec{v}_1)^2 \hat{n} \times \vec{S}_1 \cdot \vec{v}_1 + 6 \hat{n} \cdot \vec{v}_1 \vec{S}_1 \times \vec{v}_1 \cdot \vec{v}_2 - 30 \hat{n} \cdot \vec{v}_2 \hat{n} \cdot \vec{v}_1 \hat{n} \times \vec{S}_1 \cdot \vec{v}_1 + \frac{15}{4} (\hat{n} \cdot \vec{v}_2)^2 \hat{n} \times \vec{S}_1 \cdot \vec{v}_1 - \right. \\ \left. \frac{3}{2} \hat{n} \cdot \vec{v}_2 \vec{S}_1 \times \vec{v}_1 \cdot \vec{v}_2 - \frac{3}{4} \vec{v}_1 \cdot \vec{v}_1 \hat{n} \times \vec{S}_1 \cdot \vec{v}_1 + 6 \vec{v}_1 \cdot \vec{v}_2 \hat{n} \times \vec{S}_1 \cdot \vec{v}_1 - \frac{3}{4} \vec{v}_2 \cdot \vec{v}_2 \hat{n} \times \vec{S}_1 \cdot \vec{v}_1 \right) \}$$

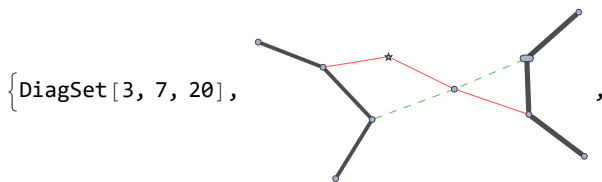

$$\frac{1}{r^3} \pi^2 G^3 m_1 m_2^2 \left( \frac{9}{4} \hat{n} \cdot \vec{a}_2 \hat{n} \times \vec{S}_1 \cdot \vec{v}_2 - \frac{3}{2} \hat{n} \cdot \vec{v}_2 \hat{n} \times \vec{S}_1 \cdot \vec{a}_2 - \frac{5}{4} \vec{S}_1 \times \vec{v}_2 \cdot \vec{a}_2 + \frac{3}{4} \hat{n} \cdot \vec{v}_2 \hat{n} \times \vec{S}_1 \cdot \vec{v}_2 \right) + \frac{1}{r^4} \pi^2 G^3 m_1 m_2^2 \\ \left( \frac{45}{16} (\hat{n} \cdot \vec{v}_2)^2 \hat{n} \times \vec{S}_1 \cdot \vec{v}_2 - \frac{3}{4} \hat{n} \cdot \vec{v}_2 \vec{S}_1 \times \vec{v}_1 \cdot \vec{v}_2 - \frac{15}{4} \hat{n} \cdot \vec{v}_1 \hat{n} \cdot \vec{v}_2 \hat{n} \times \vec{S}_1 \cdot \vec{v}_2 + \frac{3}{4} \vec{v}_1 \cdot \vec{v}_2 \hat{n} \times \vec{S}_1 \cdot \vec{v}_2 - \frac{9}{16} \vec{v}_2 \cdot \vec{v}_2 \hat{n} \times \vec{S}_1 \cdot \vec{v}_2 \right) \}$$

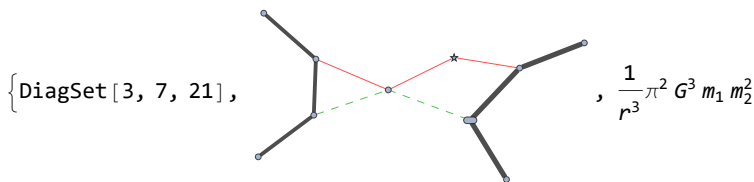

$$\left( \frac{9}{4} \hat{n} \cdot \vec{a}_2 \hat{n} \times \vec{S}_1 \cdot \vec{v}_1 + \frac{3}{2} \hat{n} \cdot \vec{v}_1 \hat{n} \times \vec{a}_2 \cdot \vec{S}_1 - \frac{5}{4} \vec{a}_2 \times \vec{S}_1 \cdot \vec{v}_1 - \frac{3}{2} \hat{n} \cdot \vec{v}_1 \hat{n} \times \vec{S}_1 \cdot \vec{v}_2 + \frac{9}{4} \hat{n} \cdot \vec{v}_2 \hat{n} \times \vec{S}_1 \cdot \vec{v}_1 - \frac{5}{4} \frac{1}{\vec{S}_1 \times \vec{v}_1 \cdot \vec{v}_2} \right) + \\ \frac{1}{r^4} \pi^2 G^3 m_1 m_2^2 \left( \frac{45}{8} (\hat{n} \cdot \vec{v}_1)^2 \hat{n} \times \vec{S}_1 \cdot \vec{v}_2 + \frac{15}{4} \hat{n} \cdot \vec{v}_1 \vec{S}_1 \times \vec{v}_1 \cdot \vec{v}_2 - \frac{15}{2} \hat{n} \cdot \vec{v}_2 \hat{n} \cdot \vec{v}_1 \hat{n} \times \vec{S}_1 \cdot \vec{v}_1 - \right. \\ \left. \frac{15}{2} \hat{n} \cdot \vec{v}_2 \hat{n} \cdot \vec{v}_1 \hat{n} \times \vec{S}_1 \cdot \vec{v}_2 + \frac{45}{4} (\hat{n} \cdot \vec{v}_2)^2 \hat{n} \times \vec{S}_1 \cdot \vec{v}_1 - 6 \hat{n} \cdot \vec{v}_2 \vec{S}_1 \times \vec{v}_1 \cdot \vec{v}_2 - \right. \\ \left. \frac{9}{8} \vec{v}_1 \cdot \vec{v}_1 \hat{n} \times \vec{S}_1 \cdot \vec{v}_2 + \frac{3}{2} \vec{v}_1 \cdot \vec{v}_2 \hat{n} \times \vec{S}_1 \cdot \vec{v}_1 + \frac{3}{2} \vec{v}_1 \cdot \vec{v}_2 \hat{n} \times \vec{S}_1 \cdot \vec{v}_2 - \frac{9}{4} \vec{v}_2 \cdot \vec{v}_2 \hat{n} \times \vec{S}_1 \cdot \vec{v}_1 \right) \}$$

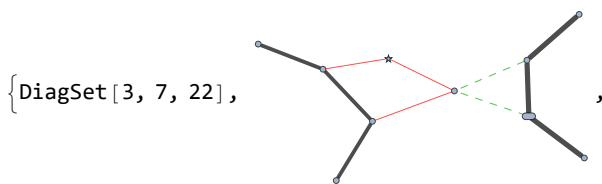

$$\frac{\pi^2 G^3 m_1 m_2^2 \left( \frac{3}{2} \hat{n} \cdot \vec{v}_2 \hat{n} \times \vec{a}_1 \cdot \vec{S}_1 - \frac{1}{2} \vec{a}_1 \times \vec{S}_1 \cdot \vec{v}_2 - \frac{3}{2} \hat{n} \cdot \vec{v}_2 \hat{n} \times \vec{S}_1 \cdot \vec{v}_1 + \frac{1}{2} \vec{S}_1 \times \vec{v}_1 \cdot \vec{v}_2 \right)}{r^3} +$$

$$\frac{1}{r^4} \pi^2 G^3 m_1 m_2^2 \left( -\frac{15}{4} (\hat{n} \cdot \vec{v}_2)^2 \hat{n} \times \vec{S}_1 \cdot \vec{v}_1 + \frac{3}{2} \hat{n} \cdot \vec{v}_2 \vec{S}_1 \times \vec{v}_1 \cdot \vec{v}_2 + \frac{15}{2} \hat{n} \cdot \vec{v}_1 \hat{n} \cdot \vec{v}_2 \hat{n} \times \vec{S}_1 \cdot \vec{v}_1 - \frac{3}{2} \hat{n} \cdot \vec{v}_1 \vec{S}_1 \times \vec{v}_1 \cdot \vec{v}_2 - \frac{3}{2} \vec{v}_1 \cdot \vec{v}_2 \hat{n} \times \vec{S}_1 \cdot \vec{v}_1 + \frac{3}{4} \vec{v}_2 \cdot \vec{v}_2 \hat{n} \times \vec{S}_1 \cdot \vec{v}_1 \right) \Big\}$$

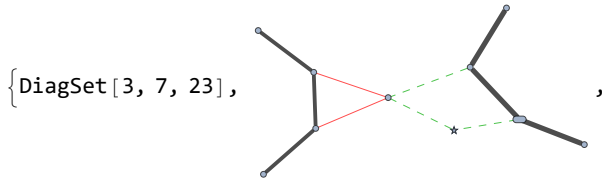

$$\frac{1}{r^3} \pi^2 G^3 m_1 m_2^2 \left( \frac{3}{4} \hat{n} \cdot \vec{a}_1 \hat{n} \times \vec{S}_1 \cdot \vec{v}_1 - \frac{1}{4} \vec{a}_1 \times \vec{S}_1 \cdot \vec{v}_1 + \frac{9}{4} \hat{n} \cdot \vec{v}_1 \hat{n} \times \vec{S}_1 \cdot \vec{v}_1 - 3 \hat{n} \cdot \vec{v}_2 \hat{n} \times \vec{S}_1 \cdot \vec{v}_1 + \vec{S}_1 \times \vec{v}_1 \cdot \vec{v}_2 \right) +$$

$$\frac{\pi^2 G^3 m_1 m_2^2 \hat{n} \times \vec{a}_1 \cdot \vec{S}_1}{r^2} + \frac{1}{r^4} \pi^2 G^3 m_1 m_2^2 \left( -\frac{15}{8} (\hat{n} \cdot \vec{v}_1)^2 \hat{n} \times \vec{S}_1 \cdot \vec{v}_1 - \frac{3}{4} \hat{n} \cdot \vec{v}_1 \vec{S}_1 \times \vec{v}_1 \cdot \vec{v}_2 + \frac{15}{4} \hat{n} \cdot \vec{v}_2 \hat{n} \cdot \vec{v}_1 \hat{n} \times \vec{S}_1 \cdot \vec{v}_1 + \frac{3}{8} \vec{v}_1 \cdot \vec{v}_1 \hat{n} \times \vec{S}_1 \cdot \vec{v}_1 - \frac{3}{4} \vec{v}_1 \cdot \vec{v}_2 \hat{n} \times \vec{S}_1 \cdot \vec{v}_1 \right) \Big\}$$

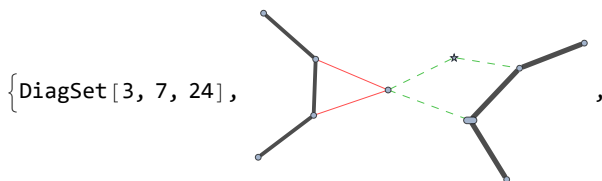

$$\frac{1}{r^3} \pi^2 G^3 m_1 m_2^2 \left( \frac{9}{4} \hat{n} \cdot \vec{a}_1 \hat{n} \times \vec{S}_1 \cdot \vec{v}_1 + \frac{9}{2} \hat{n} \cdot \vec{v}_1 \hat{n} \times \vec{a}_1 \cdot \vec{S}_1 - 3 \hat{n} \cdot \vec{v}_2 \hat{n} \times \vec{a}_1 \cdot \vec{S}_1 -$$

$$\frac{9}{4} \vec{a}_1 \times \vec{S}_1 \cdot \vec{v}_1 + \vec{a}_1 \times \vec{S}_1 \cdot \vec{v}_2 - \frac{3}{4} \hat{n} \cdot \vec{v}_1 \hat{n} \times \vec{S}_1 \cdot \vec{v}_1 \right) - \frac{\pi^2 G^3 m_1 m_2^2 \hat{n} \times \vec{a}_1 \cdot \vec{S}_1}{r^2} + \frac{1}{r^4} \pi^2 G^3 m_1 m_2^2 \left( \frac{15}{8} (\hat{n} \cdot \vec{v}_1)^2 \hat{n} \times \vec{S}_1 \cdot \vec{v}_1 + \frac{3}{4} \hat{n} \cdot \vec{v}_1 \vec{S}_1 \times \vec{v}_1 \cdot \vec{v}_2 - \frac{15}{4} \hat{n} \cdot \vec{v}_2 \hat{n} \cdot \vec{v}_1 \hat{n} \times \vec{S}_1 \cdot \vec{v}_1 - \frac{3}{8} \vec{v}_1 \cdot \vec{v}_1 \hat{n} \times \vec{S}_1 \cdot \vec{v}_1 + \frac{3}{4} \vec{v}_1 \cdot \vec{v}_2 \hat{n} \times \vec{S}_1 \cdot \vec{v}_1 \right) \Big\}$$

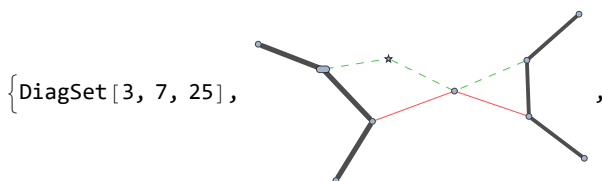

$$\frac{1}{r^3} \pi^2 G^3 m_1 m_2^2 \left( -\frac{3}{4} \hat{n} \cdot \vec{a}_2 \hat{n} \times \vec{S}_1 \cdot \vec{v}_1 - \frac{9}{2} \hat{n} \cdot \vec{v}_1 \hat{n} \times \vec{S}_1 \cdot \vec{a}_2 - \frac{5}{4} \vec{S}_1 \times \vec{v}_1 \cdot \vec{a}_2 - \frac{9}{2} \hat{n} \cdot \vec{v}_1 \hat{n} \times \vec{S}_1 \cdot \vec{v}_2 +$$

$$\frac{3}{4} \hat{n} \cdot \vec{v}_2 \hat{n} \times \vec{S}_1 \cdot \vec{v}_1 + 9 \hat{n} \cdot \vec{v}_2 \hat{n} \times \vec{S}_1 \cdot \vec{v}_2 - \frac{7}{4} \vec{S}_1 \times \vec{v}_1 \cdot \vec{v}_2 \right) + \frac{3 \pi^2 G^3 m_1 m_2^2 \hat{n} \times \vec{S}_1 \cdot \vec{a}_2}{r^2} + \frac{1}{r^4} \pi^2 G^3 m_1 m_2^2 \left( \frac{45}{8} (\hat{n} \cdot \vec{v}_1)^2 \hat{n} \times \vec{S}_1 \cdot \vec{v}_2 + \frac{9}{4} \hat{n} \cdot \vec{v}_1 \vec{S}_1 \times \vec{v}_1 \cdot \vec{v}_2 - \frac{45}{2} \hat{n} \cdot \vec{v}_2 \hat{n} \cdot \vec{v}_1 \hat{n} \times \vec{S}_1 \cdot \vec{v}_2 - \frac{15}{4} (\hat{n} \cdot \vec{v}_2)^2 \hat{n} \times \vec{S}_1 \cdot \vec{v}_1 - 3 \hat{n} \cdot \vec{v}_2 \vec{S}_1 \times \vec{v}_1 \cdot \vec{v}_2 - \frac{9}{8} \vec{v}_1 \cdot \vec{v}_1 \hat{n} \times \vec{S}_1 \cdot \vec{v}_2 + \frac{9}{2} \vec{v}_1 \cdot \vec{v}_2 \hat{n} \times \vec{S}_1 \cdot \vec{v}_2 + \frac{3}{4} \vec{v}_2 \cdot \vec{v}_2 \hat{n} \times \vec{S}_1 \cdot \vec{v}_1 \right) \Big\}$$



{DiagSet[3, 7, 26],

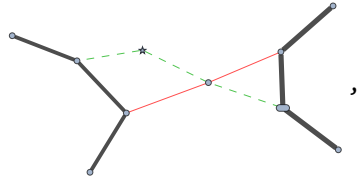

,

$$\frac{1}{r^3} \pi^2 G^3 m_1 m_2^2 \left( \frac{9}{4} \hat{n} \cdot \vec{a}_2 \hat{n} \times \vec{S}_1 \cdot \vec{v}_2 - \frac{3}{2} \hat{n} \cdot \vec{v}_1 \hat{n} \times \vec{S}_1 \cdot \vec{a}_2 - \frac{3}{2} \hat{n} \cdot \vec{v}_2 \hat{n} \times \vec{S}_1 \cdot \vec{a}_2 - \frac{1}{2} \vec{S}_1 \times \vec{v}_1 \cdot \vec{a}_2 - \frac{5}{4} \vec{S}_1 \times \vec{v}_2 \cdot \vec{a}_2 + \frac{3}{4} \hat{n} \cdot \vec{v}_2 \hat{n} \times \vec{S}_1 \cdot \vec{v}_2 \right) + \frac{\pi^2 G^3 m_1 m_2^2 \hat{n} \times \vec{S}_1 \cdot \vec{a}_2}{2 r^2} + \frac{1}{r^4} \pi^2 G^3 m_1 m_2^2 \left( \frac{15}{16} (\hat{n} \cdot \vec{v}_2)^2 \hat{n} \times \vec{S}_1 \cdot \vec{v}_2 - \frac{3}{4} \hat{n} \cdot \vec{v}_2 \vec{S}_1 \times \vec{v}_1 \cdot \vec{v}_2 - \frac{15}{4} \hat{n} \cdot \vec{v}_1 \hat{n} \cdot \vec{v}_2 \hat{n} \times \vec{S}_1 \cdot \vec{v}_2 + \frac{3}{4} \vec{v}_1 \cdot \vec{v}_2 \hat{n} \times \vec{S}_1 \cdot \vec{v}_2 - \frac{3}{16} \vec{v}_2 \cdot \vec{v}_2 \hat{n} \times \vec{S}_1 \cdot \vec{v}_2 \right) \}$$

{DiagSet[3, 8, 1],

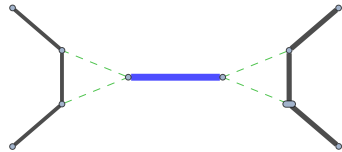

,

$$\frac{\pi^2 G^3 m_1 m_2^2 \left( -\frac{15}{4} (\hat{n} \cdot \vec{v}_2)^2 \hat{n} \times \vec{S}_1 \cdot \vec{v}_1 + \frac{3}{2} \hat{n} \cdot \vec{v}_2 \vec{S}_1 \times \vec{v}_1 \cdot \vec{v}_2 + \frac{3}{4} \vec{v}_2 \cdot \vec{v}_2 \hat{n} \times \vec{S}_1 \cdot \vec{v}_1 \right)}{r^4} \}$$

{DiagSet[3, 8, 2],

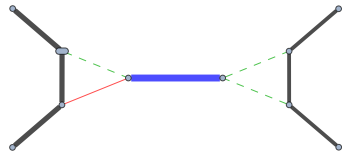

$$, \frac{3 \pi^2 G^3 m_1 m_2^2 \hat{n} \cdot \vec{v}_2 \hat{n} \times \vec{S}_1 \cdot \vec{v}_2}{2 r^3} \}$$

{DiagSet[3, 8, 3],

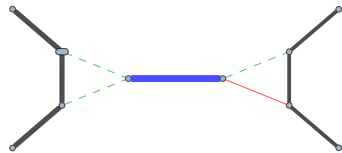

$$, \frac{\pi^2 G^3 m_1 m_2^2 \left( -\frac{3}{2} \hat{n} \cdot \vec{v}_1 \hat{n} \times \vec{S}_1 \cdot \vec{a}_2 - \frac{1}{2} \vec{S}_1 \times \vec{v}_1 \cdot \vec{a}_2 \right)}{r^3} \}$$

{DiagSet[3, 8, 4],

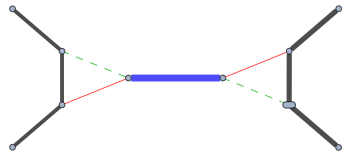

$$, \frac{\pi^2 G^3 m_1 m_2^2 \hat{n} \times \vec{S}_1 \cdot \vec{a}_2}{2 r^2} \}$$

{DiagSet[3, 8, 5],

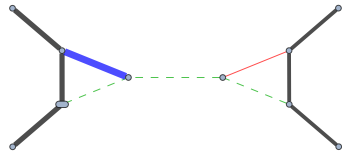

,

$$\frac{\pi^2 G^3 m_1 m_2^2 \left( \frac{45}{2} (\hat{n} \cdot \vec{v}_1)^2 \hat{n} \times \vec{S}_1 \cdot \vec{v}_2 + 9 \hat{n} \cdot \vec{v}_1 \vec{S}_1 \times \vec{v}_1 \cdot \vec{v}_2 - \frac{9}{2} \vec{v}_1 \cdot \vec{v}_1 \hat{n} \times \vec{S}_1 \cdot \vec{v}_2 \right)}{r^4} \}$$

{DiagSet[3, 8, 6],

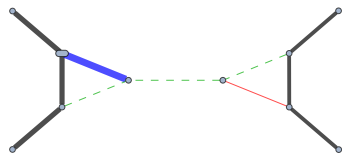

, 0}

$$\left\{ \text{DiagSet}[3, 8, 7], \right.$$
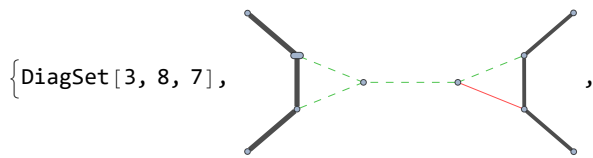

$$\frac{1}{r^3} \pi^2 G^3 m_1 m_2^2 \left( \frac{9}{2} \hat{n} \cdot \vec{v}_1 \hat{n} \times \vec{a}_2 \cdot \vec{S}_1 + \frac{9}{2} \hat{n} \cdot \vec{v}_2 \hat{n} \times \vec{a}_1 \cdot \vec{S}_1 - \frac{3}{2} \vec{a}_1 \times \vec{S}_1 \cdot \vec{v}_2 - \frac{3}{2} \vec{a}_2 \times \vec{S}_1 \cdot \vec{v}_1 + 6 \hat{n} \cdot \vec{v}_1 \hat{n} \times \vec{S}_1 \cdot \vec{v}_2 - \frac{3}{2} \hat{n} \cdot \vec{v}_2 \hat{n} \times \vec{S}_1 \cdot \vec{v}_1 + \frac{5}{2} \vec{S}_1 \times \vec{v}_1 \cdot \vec{v}_2 \right) + \frac{1}{r^4} \pi^2 G^3 m_1 m_2^2 \left( -\frac{45}{2} (\hat{n} \cdot \vec{v}_1)^2 \hat{n} \times \vec{S}_1 \cdot \vec{v}_2 - \frac{21}{2} \hat{n} \cdot \vec{v}_1 \vec{S}_1 \times \vec{v}_1 \cdot \vec{v}_2 + \frac{15}{2} \hat{n} \cdot \vec{v}_2 \hat{n} \cdot \vec{v}_1 \hat{n} \times \vec{S}_1 \cdot \vec{v}_1 - \frac{45}{2} \hat{n} \cdot \vec{v}_2 \hat{n} \cdot \vec{v}_1 \hat{n} \times \vec{S}_1 \cdot \vec{v}_2 - \frac{9}{2} \hat{n} \cdot \vec{v}_2 \vec{S}_1 \times \vec{v}_1 \cdot \vec{v}_2 + \frac{9}{2} \vec{v}_1 \cdot \vec{v}_1 \hat{n} \times \vec{S}_1 \cdot \vec{v}_2 - \frac{3}{2} \vec{v}_1 \cdot \vec{v}_2 \hat{n} \times \vec{S}_1 \cdot \vec{v}_1 + \frac{9}{2} \vec{v}_1 \cdot \vec{v}_2 \hat{n} \times \vec{S}_1 \cdot \vec{v}_2 \right) \}$$

$$\left\{ \text{DiagSet}[3, 8, 8], \right.$$
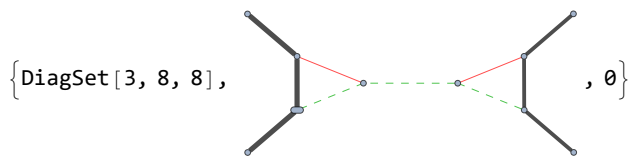

, 0}

$$\left\{ \text{DiagSet}[3, 8, 9], \right.$$
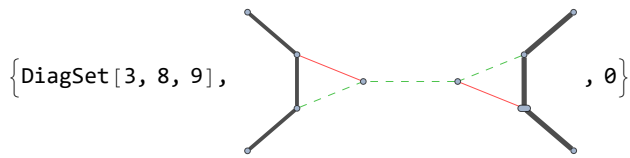

, 0}

$$\left\{ \text{DiagSet}[3, 8, 10], \right.$$
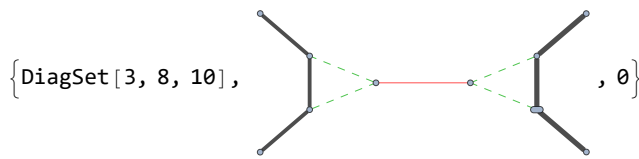

, 0}

$$\left\{ \text{DiagSet}[3, 8, 11], \right.$$
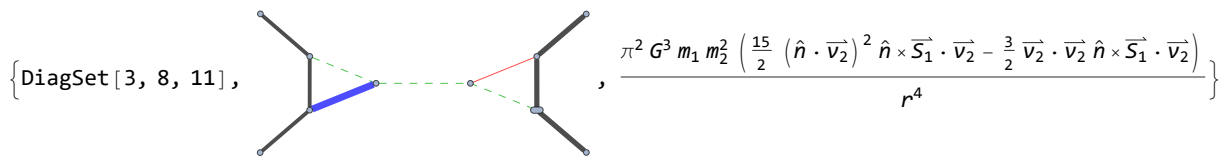

,  $\frac{\pi^2 G^3 m_1 m_2^2 \left( \frac{15}{2} (\hat{n} \cdot \vec{v}_2)^2 \hat{n} \times \vec{S}_1 \cdot \vec{v}_2 - \frac{3}{2} \vec{v}_2 \cdot \vec{v}_2 \hat{n} \times \vec{S}_1 \cdot \vec{v}_2 \right)}{r^4} \}$ 

$$\left\{ \text{DiagSet}[3, 8, 12], \right.$$
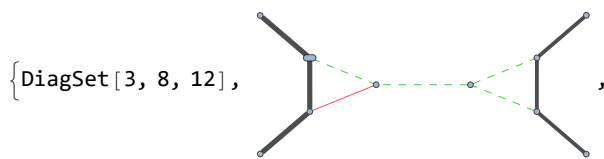

,

$$\frac{\pi^2 G^3 m_1 m_2^2 \left( -3 \hat{n} \cdot \vec{v}_2 \hat{n} \times \vec{S}_1 \cdot \vec{a}_2 - (\vec{S}_1 \times \vec{v}_2 \cdot \vec{a}_2) + \frac{3}{2} \hat{n} \cdot \vec{v}_2 \hat{n} \times \vec{S}_1 \cdot \vec{v}_2 \right)}{r^3} + \frac{1}{r^4} \pi^2 G^3 m_1 m_2^2 \left( -\frac{15}{2} (\hat{n} \cdot \vec{v}_2)^2 \hat{n} \times \vec{S}_1 \cdot \vec{v}_2 - \frac{3}{2} \hat{n} \cdot \vec{v}_2 \vec{S}_1 \times \vec{v}_1 \cdot \vec{v}_2 - \frac{15}{2} \hat{n} \cdot \vec{v}_1 \hat{n} \cdot \vec{v}_2 \hat{n} \times \vec{S}_1 \cdot \vec{v}_2 + \frac{3}{2} \vec{v}_1 \cdot \vec{v}_2 \hat{n} \times \vec{S}_1 \cdot \vec{v}_2 + \frac{3}{2} \vec{v}_2 \cdot \vec{v}_2 \hat{n} \times \vec{S}_1 \cdot \vec{v}_2 \right) \}$$

$$\left\{ \text{DiagSet}[3, 8, 13], \right.$$
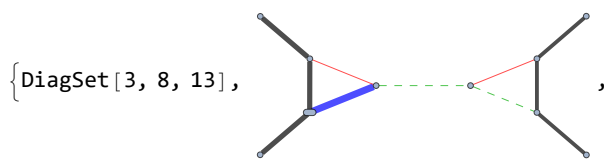

,

$$\frac{\pi^2 G^3 m_1 m_2^2 \left( \frac{3}{2} \hat{n} \cdot \vec{v}_1 \hat{n} \times \vec{S}_1 \cdot \vec{a}_2 + \frac{1}{2} \vec{S}_1 \times \vec{v}_1 \cdot \vec{a}_2 \right)}{r^3} + \frac{1}{r^4} \pi^2 G^3 m_1 m_2^2 \left( -\frac{15}{2} (\hat{n} \cdot \vec{v}_1)^2 \hat{n} \times \vec{S}_1 \cdot \vec{v}_2 - 3 \hat{n} \cdot \vec{v}_1 \vec{S}_1 \times \vec{v}_1 \cdot \vec{v}_2 + \right.$$

$$\frac{15}{2} \hat{n} \cdot \vec{v}_2 \hat{n} \cdot \vec{v}_1 \hat{n} \times \vec{S}_1 \cdot \vec{v}_2 + \frac{3}{2} \hat{n} \cdot \vec{v}_2 \vec{S}_1 \times \vec{v}_1 \cdot \vec{v}_2 + \frac{3}{2} \vec{v}_1 \cdot \vec{v}_1 \hat{n} \times \vec{S}_1 \cdot \vec{v}_2 - \frac{3}{2} \vec{v}_1 \cdot \vec{v}_2 \hat{n} \times \vec{S}_1 \cdot \vec{v}_2 \Bigg\}$$

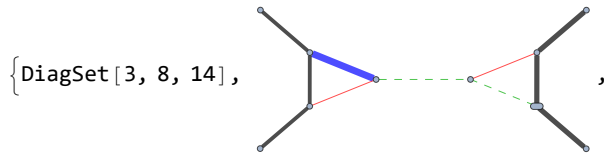

$$\frac{1}{r^4} \pi^2 G^3 m_1 m_2^2 \left( -\frac{15}{2} (\hat{n} \cdot \vec{v}_2)^2 \hat{n} \times \vec{S}_1 \cdot \vec{v}_2 + \frac{3}{2} \hat{n} \cdot \vec{v}_2 \vec{S}_1 \times \vec{v}_1 \cdot \vec{v}_2 + \frac{15}{2} \hat{n} \cdot \vec{v}_1 \hat{n} \cdot \vec{v}_2 \hat{n} \times \vec{S}_1 \cdot \vec{v}_2 - \right.$$

$$\left. \frac{3}{2} \vec{v}_1 \cdot \vec{v}_2 \hat{n} \times \vec{S}_1 \cdot \vec{v}_2 + \frac{3}{2} \vec{v}_2 \cdot \vec{v}_2 \hat{n} \times \vec{S}_1 \cdot \vec{v}_2 \right) - \frac{3 \pi^2 G^3 m_1 m_2^2 \hat{n} \cdot \vec{v}_2 \hat{n} \times \vec{S}_1 \cdot \vec{v}_2}{2 r^3} \Bigg\}$$

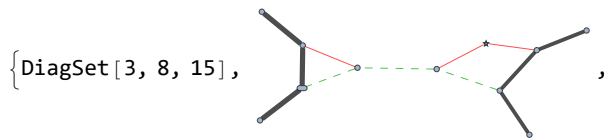

$$\frac{\pi^2 G^3 m_1 m_2^2 \left( -\frac{3}{4} \hat{n} \cdot \vec{a}_2 \hat{n} \times \vec{S}_1 \cdot \vec{v}_2 + \frac{1}{4} \vec{S}_1 \times \vec{v}_2 \cdot \vec{a}_2 - \frac{3}{4} \hat{n} \cdot \vec{v}_2 \hat{n} \times \vec{S}_1 \cdot \vec{v}_2 \right)}{r^3} + \frac{1}{r^4} \pi^2 G^3 m_1 m_2^2 \left( -\frac{45}{16} (\hat{n} \cdot \vec{v}_2)^2 \hat{n} \times \vec{S}_1 \cdot \vec{v}_2 + \right.$$

$$\left. \frac{3}{4} \hat{n} \cdot \vec{v}_2 \vec{S}_1 \times \vec{v}_1 \cdot \vec{v}_2 + \frac{15}{4} \hat{n} \cdot \vec{v}_1 \hat{n} \cdot \vec{v}_2 \hat{n} \times \vec{S}_1 \cdot \vec{v}_2 - \frac{3}{4} \vec{v}_1 \cdot \vec{v}_2 \hat{n} \times \vec{S}_1 \cdot \vec{v}_2 + \frac{9}{16} \vec{v}_2 \cdot \vec{v}_2 \hat{n} \times \vec{S}_1 \cdot \vec{v}_2 \right) \Bigg\}$$

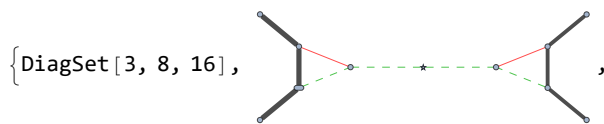

$$\frac{\pi^2 G^3 m_1 m_2^2 \left( \frac{3}{2} \hat{n} \cdot \vec{v}_1 \hat{n} \times \vec{S}_1 \cdot \vec{a}_2 + \frac{1}{2} \vec{S}_1 \times \vec{v}_1 \cdot \vec{a}_2 - \frac{3}{2} \hat{n} \cdot \vec{v}_2 \hat{n} \times \vec{S}_1 \cdot \vec{v}_2 \right)}{r^3} - \frac{\pi^2 G^3 m_1 m_2^2 \hat{n} \times \vec{S}_1 \cdot \vec{a}_2}{2 r^2} +$$

$$\frac{1}{r^4} \pi^2 G^3 m_1 m_2^2 \left( \frac{3}{2} \hat{n} \cdot \vec{v}_2 \vec{S}_1 \times \vec{v}_1 \cdot \vec{v}_2 + \frac{15}{2} \hat{n} \cdot \vec{v}_1 \hat{n} \cdot \vec{v}_2 \hat{n} \times \vec{S}_1 \cdot \vec{v}_2 - \frac{3}{2} \vec{v}_1 \cdot \vec{v}_2 \hat{n} \times \vec{S}_1 \cdot \vec{v}_2 \right) \Bigg\}$$

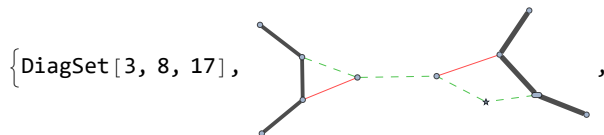

$$\frac{1}{r^3} \pi^2 G^3 m_1 m_2^2 \left( \frac{3}{4} \hat{n} \cdot \vec{a}_2 \hat{n} \times \vec{S}_1 \cdot \vec{v}_1 + \frac{9}{2} \hat{n} \cdot \vec{v}_1 \hat{n} \times \vec{S}_1 \cdot \vec{a}_2 + \frac{5}{4} \vec{S}_1 \times \vec{v}_1 \cdot \vec{a}_2 + \frac{9}{2} \hat{n} \cdot \vec{v}_1 \hat{n} \times \vec{S}_1 \cdot \vec{v}_2 - \right.$$

$$\left. \frac{3}{4} \hat{n} \cdot \vec{v}_2 \hat{n} \times \vec{S}_1 \cdot \vec{v}_1 - 9 \hat{n} \cdot \vec{v}_2 \hat{n} \times \vec{S}_1 \cdot \vec{v}_2 + \frac{7}{4} \vec{S}_1 \times \vec{v}_1 \cdot \vec{v}_2 \right) - \frac{3 \pi^2 G^3 m_1 m_2^2 \hat{n} \times \vec{S}_1 \cdot \vec{a}_2}{r^2} + \frac{1}{r^4}$$

$$\pi^2 G^3 m_1 m_2^2 \left( -\frac{45}{8} (\hat{n} \cdot \vec{v}_1)^2 \hat{n} \times \vec{S}_1 \cdot \vec{v}_2 - \frac{9}{4} \hat{n} \cdot \vec{v}_1 \vec{S}_1 \times \vec{v}_1 \cdot \vec{v}_2 + \frac{45}{2} \hat{n} \cdot \vec{v}_2 \hat{n} \cdot \vec{v}_1 \hat{n} \times \vec{S}_1 \cdot \vec{v}_2 + \frac{15}{4} (\hat{n} \cdot \vec{v}_2)^2 \hat{n} \times \vec{S}_1 \cdot \vec{v}_1 + \right.$$

$$\left. 3 \hat{n} \cdot \vec{v}_2 \vec{S}_1 \times \vec{v}_1 \cdot \vec{v}_2 + \frac{9}{8} \vec{v}_1 \cdot \vec{v}_1 \hat{n} \times \vec{S}_1 \cdot \vec{v}_2 - \frac{9}{2} \vec{v}_1 \cdot \vec{v}_2 \hat{n} \times \vec{S}_1 \cdot \vec{v}_2 - \frac{3}{4} \vec{v}_2 \cdot \vec{v}_2 \hat{n} \times \vec{S}_1 \cdot \vec{v}_1 \right) \Bigg\}$$

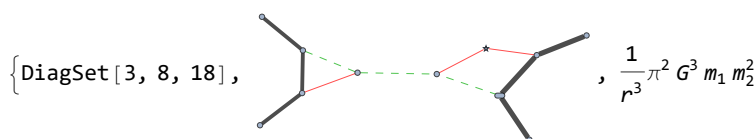

$$\left( -\frac{9}{4} \hat{n} \cdot \vec{a}_2 \hat{n} \times \vec{S}_1 \cdot \vec{v}_1 - \frac{3}{2} \hat{n} \cdot \vec{v}_1 \hat{n} \times \vec{a}_2 \cdot \vec{S}_1 + \frac{5}{4} \vec{a}_2 \times \vec{S}_1 \cdot \vec{v}_1 + \frac{3}{2} \hat{n} \cdot \vec{v}_1 \hat{n} \times \vec{S}_1 \cdot \vec{v}_2 - \frac{9}{4} \hat{n} \cdot \vec{v}_2 \hat{n} \times \vec{S}_1 \cdot \vec{v}_1 + \frac{5}{4} \vec{S}_1 \times \vec{v}_1 \cdot \vec{v}_2 \right) +$$

$$\frac{1}{r^4} \pi^2 G^3 m_1 m_2^2 \left( -\frac{45}{8} (\hat{n} \cdot \vec{v}_1)^2 \hat{n} \times \vec{S}_1 \cdot \vec{v}_2 - \frac{15}{4} \hat{n} \cdot \vec{v}_1 \vec{S}_1 \times \vec{v}_1 \cdot \vec{v}_2 + \frac{15}{2} \hat{n} \cdot \vec{v}_2 \hat{n} \cdot \vec{v}_1 \hat{n} \times \vec{S}_1 \cdot \vec{v}_1 + \right.$$

$$\frac{15}{2} \hat{n} \cdot \vec{v}_2 \hat{n} \cdot \vec{v}_1 \hat{n} \times \vec{S}_1 \cdot \vec{v}_2 - \frac{45}{4} (\hat{n} \cdot \vec{v}_2)^2 \hat{n} \times \vec{S}_1 \cdot \vec{v}_1 + 6 \hat{n} \cdot \vec{v}_2 \vec{S}_1 \times \vec{v}_1 \cdot \vec{v}_2 +$$

$$\left. \frac{9}{8} \vec{v}_1 \cdot \vec{v}_1 \hat{n} \times \vec{S}_1 \cdot \vec{v}_2 - \frac{3}{2} \vec{v}_1 \cdot \vec{v}_2 \hat{n} \times \vec{S}_1 \cdot \vec{v}_1 - \frac{3}{2} \vec{v}_1 \cdot \vec{v}_2 \hat{n} \times \vec{S}_1 \cdot \vec{v}_2 + \frac{9}{4} \vec{v}_2 \cdot \vec{v}_2 \hat{n} \times \vec{S}_1 \cdot \vec{v}_1 \right) \Bigg\}$$

$$\left\{ \text{DiagSet}[3, 8, 19], \right.$$
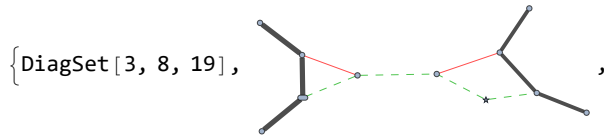

$$,$$

$$\frac{1}{r^3} \pi^2 G^3 m_1 m_2^2 \left( -\frac{3}{4} \hat{n} \cdot \vec{a}_2 \hat{n} \times \vec{S}_1 \cdot \vec{v}_2 - \frac{3}{2} \hat{n} \cdot \vec{v}_1 \hat{n} \times \vec{a}_2 \cdot \vec{S}_1 + \frac{1}{2} \vec{a}_2 \times \vec{S}_1 \cdot \vec{v}_1 + \frac{1}{4} \vec{a}_2 \times \vec{S}_1 \cdot \vec{v}_2 - \frac{3}{4} \hat{n} \cdot \vec{v}_2 \hat{n} \times \vec{S}_1 \cdot \vec{v}_2 \right) +$$

$$\frac{\pi^2 G^3 m_1 m_2^2 \hat{n} \times \vec{a}_2 \cdot \vec{S}_1}{2 r^2} + \frac{1}{r^4} \pi^2 G^3 m_1 m_2^2 \left( -\frac{15}{16} (\hat{n} \cdot \vec{v}_2)^2 \hat{n} \times \vec{S}_1 \cdot \vec{v}_2 + \right.$$

$$\left. \frac{3}{4} \hat{n} \cdot \vec{v}_2 \vec{S}_1 \times \vec{v}_1 \cdot \vec{v}_2 + \frac{15}{4} \hat{n} \cdot \vec{v}_1 \hat{n} \cdot \vec{v}_2 \hat{n} \times \vec{S}_1 \cdot \vec{v}_2 - \frac{3}{4} \vec{v}_1 \cdot \vec{v}_2 \hat{n} \times \vec{S}_1 \cdot \vec{v}_2 + \frac{3}{16} \vec{v}_2 \cdot \vec{v}_2 \hat{n} \times \vec{S}_1 \cdot \vec{v}_2 \right) \Bigg\}$$

$$\left\{ \text{DiagSet}[3, 8, 20], \right.$$
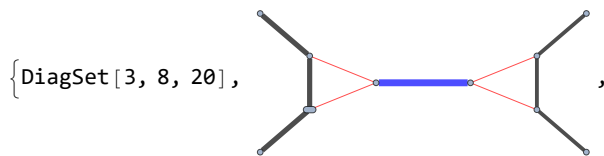

$$,$$

$$\frac{\pi^2 G^3 m_1 m_2^2 \left( \frac{3}{16} \hat{n} \cdot \vec{v}_1 \hat{n} \times \vec{S}_1 \cdot \vec{a}_1 + \frac{1}{16} \vec{S}_1 \times \vec{v}_1 \cdot \vec{a}_1 + \frac{3}{16} \hat{n} \cdot \vec{v}_1 \hat{n} \times \vec{S}_1 \cdot \vec{v}_1 \right)}{r^3} + \frac{1}{r^4} \pi^2 G^3 m_1 m_2^2 \left( -\frac{15}{32} (\hat{n} \cdot \vec{v}_1)^2 \hat{n} \times \vec{S}_1 \cdot \vec{v}_1 - \right.$$

$$\left. \frac{15}{32} (\hat{n} \cdot \vec{v}_2)^2 \hat{n} \times \vec{S}_1 \cdot \vec{v}_1 + \frac{3}{16} \hat{n} \cdot \vec{v}_2 \vec{S}_1 \times \vec{v}_1 \cdot \vec{v}_2 + \frac{3}{32} \vec{v}_1 \cdot \vec{v}_1 \hat{n} \times \vec{S}_1 \cdot \vec{v}_1 + \frac{3}{32} \vec{v}_2 \cdot \vec{v}_2 \hat{n} \times \vec{S}_1 \cdot \vec{v}_1 \right) \Bigg\}$$

$$\left\{ \text{DiagSet}[3, 8, 21], \right.$$
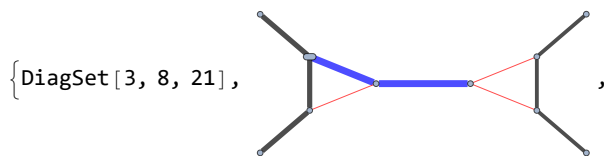

$$,$$

$$\frac{\pi^2 G^3 m_1 m_2^2 \left( \frac{3}{8} \hat{n} \cdot \vec{v}_2 \hat{n} \times \vec{a}_1 \cdot \vec{S}_1 - \frac{1}{8} \vec{a}_1 \times \vec{S}_1 \cdot \vec{v}_2 - \frac{3}{8} \hat{n} \cdot \vec{v}_2 \hat{n} \times \vec{S}_1 \cdot \vec{v}_1 + \frac{1}{8} \vec{S}_1 \times \vec{v}_1 \cdot \vec{v}_2 \right)}{r^3} +$$

$$\frac{1}{r^4} \pi^2 G^3 m_1 m_2^2 \left( -\frac{3}{8} \hat{n} \cdot \vec{v}_1 \vec{S}_1 \times \vec{v}_1 \cdot \vec{v}_2 + \frac{15}{8} \hat{n} \cdot \vec{v}_2 \hat{n} \cdot \vec{v}_1 \hat{n} \times \vec{S}_1 \cdot \vec{v}_1 - \frac{3}{8} \vec{v}_1 \cdot \vec{v}_2 \hat{n} \times \vec{S}_1 \cdot \vec{v}_1 \right) \Bigg\}$$

$$\left\{ \text{DiagSet}[3, 8, 22], \right.$$
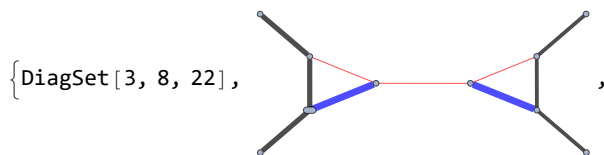

$$,$$

$$\frac{\pi^2 G^3 m_1 m_2^2 \left( \frac{15}{8} (\hat{n} \cdot \vec{v}_2)^2 \hat{n} \times \vec{S}_1 \cdot \vec{v}_1 - \frac{3}{4} \hat{n} \cdot \vec{v}_2 \vec{S}_1 \times \vec{v}_1 \cdot \vec{v}_2 - \frac{3}{8} \vec{v}_2 \cdot \vec{v}_2 \hat{n} \times \vec{S}_1 \cdot \vec{v}_1 \right)}{r^4} \Bigg\}$$

$$\left\{ \text{DiagSet}[3, 8, 23], \right. , \left. \emptyset \right\}$$

$$\left\{ \text{DiagSet}[3, 8, 24], \right. , \left. \right\}$$

$$\frac{\pi^2 G^3 m_1 m_2^2 \left( -\frac{15}{2} (\hat{n} \cdot \vec{v}_2)^2 \hat{n} \times \vec{S}_1 \cdot \vec{v}_1 + 3 \hat{n} \cdot \vec{v}_2 \vec{S}_1 \times \vec{v}_1 \cdot \vec{v}_2 + \frac{3}{2} \vec{v}_2 \cdot \vec{v}_2 \hat{n} \times \vec{S}_1 \cdot \vec{v}_1 \right)}{r^4}$$

$$\left\{ \text{DiagSet}[3, 8, 25], \right. , \left. \frac{\pi^2 G^3 m_1 m_2^2 \left( \frac{15}{64} (\hat{n} \cdot \vec{v}_1)^2 \hat{n} \times \vec{S}_1 \cdot \vec{v}_1 - \frac{3}{64} \vec{v}_1 \cdot \vec{v}_1 \hat{n} \times \vec{S}_1 \cdot \vec{v}_1 \right)}{r^4} \right\}$$

$$\left\{ \text{DiagSet}[3, 8, 26], \right. , \left. \right\}$$

$$\frac{1}{r^3} \pi^2 G^3 m_1 m_2^2 \left( -\frac{15}{32} \hat{n} \cdot \vec{a}_1 \hat{n} \times \vec{S}_1 \cdot \vec{v}_1 + \frac{9}{32} \hat{n} \cdot \vec{v}_1 \hat{n} \times \vec{S}_1 \cdot \vec{a}_1 + \frac{1}{4} \vec{S}_1 \times \vec{v}_1 \cdot \vec{a}_1 - \frac{3}{32} \hat{n} \cdot \vec{v}_1 \hat{n} \times \vec{S}_1 \cdot \vec{v}_1 \right) + \frac{1}{r^4} \pi^2 G^3 m_1 m_2^2$$

$$\left( \frac{15}{16} (\hat{n} \cdot \vec{v}_1)^2 \hat{n} \times \vec{S}_1 \cdot \vec{v}_1 + \frac{3}{4} \hat{n} \cdot \vec{v}_1 \vec{S}_1 \times \vec{v}_1 \cdot \vec{v}_2 - \frac{15}{4} \hat{n} \cdot \vec{v}_2 \hat{n} \cdot \vec{v}_1 \hat{n} \times \vec{S}_1 \cdot \vec{v}_1 - \frac{3}{16} \vec{v}_1 \cdot \vec{v}_1 \hat{n} \times \vec{S}_1 \cdot \vec{v}_1 + \frac{3}{4} \vec{v}_1 \cdot \vec{v}_2 \hat{n} \times \vec{S}_1 \cdot \vec{v}_1 \right) \}$$

$$\left\{ \text{DiagSet}[3, 8, 27], \right. , \left. \right\}$$

$$\frac{\pi^2 G^3 m_1 m_2^2 \left( -\frac{3}{32} \hat{n} \cdot \vec{a}_1 \hat{n} \times \vec{S}_1 \cdot \vec{v}_1 - \frac{3}{32} \hat{n} \cdot \vec{v}_1 \hat{n} \times \vec{S}_1 \cdot \vec{a}_1 + \frac{9}{32} \hat{n} \cdot \vec{v}_1 \hat{n} \times \vec{S}_1 \cdot \vec{v}_1 \right)}{r^3} + \frac{1}{r^4} \pi^2 G^3 m_1 m_2^2 \left( -\frac{75}{64} (\hat{n} \cdot \vec{v}_1)^2 \hat{n} \times \vec{S}_1 \cdot \vec{v}_1 - \right.$$

$$\left. \frac{3}{8} \hat{n} \cdot \vec{v}_1 \vec{S}_1 \times \vec{v}_1 \cdot \vec{v}_2 + \frac{15}{8} \hat{n} \cdot \vec{v}_2 \hat{n} \cdot \vec{v}_1 \hat{n} \times \vec{S}_1 \cdot \vec{v}_1 + \frac{15}{64} \vec{v}_1 \cdot \vec{v}_1 \hat{n} \times \vec{S}_1 \cdot \vec{v}_1 - \frac{3}{8} \vec{v}_1 \cdot \vec{v}_2 \hat{n} \times \vec{S}_1 \cdot \vec{v}_1 \right) \}$$

$$\left\{ \text{DiagSet}[3, 8, 28], \right. , \left. \right\}$$

$$\frac{1}{r^3} \pi^2 G^3 m_1 m_2^2 \left( \frac{3}{32} \hat{n} \cdot \vec{a}_1 \hat{n} \times \vec{S}_1 \cdot \vec{v}_1 - \frac{33}{32} \hat{n} \cdot \vec{v}_1 \hat{n} \times \vec{S}_1 \cdot \vec{a}_1 - \frac{3}{8} \vec{S}_1 \times \vec{v}_1 \cdot \vec{a}_1 - \frac{15}{16} \hat{n} \cdot \vec{v}_1 \hat{n} \times \vec{S}_1 \cdot \vec{v}_1 \right) +$$

$$\frac{\pi^2 G^3 m_1 m_2^2 \hat{n} \times \vec{S}_1 \cdot \vec{a}_1}{8 r^2} + \frac{1}{r^4} \pi^2 G^3 m_1 m_2^2 \left( \frac{135}{64} (\hat{n} \cdot \vec{v}_1)^2 \hat{n} \times \vec{S}_1 \cdot \vec{v}_1 - \right.$$

$$\left. \frac{15}{64} (\hat{n} \cdot \vec{v}_2)^2 \hat{n} \times \vec{S}_1 \cdot \vec{v}_1 + \frac{3}{32} \hat{n} \cdot \vec{v}_2 \vec{S}_1 \times \vec{v}_1 \cdot \vec{v}_2 - \frac{27}{64} \vec{v}_1 \cdot \vec{v}_1 \hat{n} \times \vec{S}_1 \cdot \vec{v}_1 + \frac{3}{64} \vec{v}_2 \cdot \vec{v}_2 \hat{n} \times \vec{S}_1 \cdot \vec{v}_1 \right) \}$$

$$\left\{ \text{DiagSet}[3, 8, 29], \right.$$

$$,$$

$$\frac{\pi^2 G^3 m_1 m_2^2 \left( \frac{15}{4} (\hat{n} \cdot \vec{v}_2)^2 \hat{n} \times \vec{S}_1 \cdot \vec{v}_1 - \frac{3}{2} \hat{n} \cdot \vec{v}_2 \vec{S}_1 \times \vec{v}_1 \cdot \vec{v}_2 - \frac{3}{4} \vec{v}_2 \cdot \vec{v}_2 \hat{n} \times \vec{S}_1 \cdot \vec{v}_1 \right)}{r^4} \Bigg\}$$

$$\left\{ \text{DiagSet}[3, 8, 30], \right.$$

$$,$$

$$\frac{\pi^2 G^3 m_1 m_2^2 \left( -\frac{3}{16} \hat{n} \cdot \vec{a}_1 \hat{n} \times \vec{S}_1 \cdot \vec{v}_1 - \frac{3}{16} \hat{n} \cdot \vec{v}_1 \hat{n} \times \vec{S}_1 \cdot \vec{a}_1 - \frac{3}{16} \hat{n} \cdot \vec{v}_1 \hat{n} \times \vec{S}_1 \cdot \vec{v}_1 \right)}{r^3} + \frac{1}{r^4} \pi^2 G^3 m_1 m_2^2$$

$$\left( \frac{15}{16} (\hat{n} \cdot \vec{v}_1)^2 \hat{n} \times \vec{S}_1 \cdot \vec{v}_1 + \frac{15}{64} (\hat{n} \cdot \vec{v}_2)^2 \hat{n} \times \vec{S}_1 \cdot \vec{v}_1 - \frac{3}{32} \hat{n} \cdot \vec{v}_2 \vec{S}_1 \times \vec{v}_1 \cdot \vec{v}_2 - \frac{3}{16} \vec{v}_1 \cdot \vec{v}_1 \hat{n} \times \vec{S}_1 \cdot \vec{v}_1 - \frac{3}{64} \vec{v}_2 \cdot \vec{v}_2 \hat{n} \times \vec{S}_1 \cdot \vec{v}_1 \right) \Bigg\}$$

$$\left\{ \text{DiagSet}[3, 8, 31], \right.$$

$$,$$

$$\frac{\pi^2 G^3 m_1 m_2^2 \left( \frac{3}{8} \hat{n} \cdot \vec{a}_1 \hat{n} \times \vec{S}_1 \cdot \vec{v}_1 + \frac{3}{8} \hat{n} \cdot \vec{v}_1 \hat{n} \times \vec{S}_1 \cdot \vec{a}_1 + \frac{3}{8} \hat{n} \cdot \vec{v}_1 \hat{n} \times \vec{S}_1 \cdot \vec{v}_1 \right)}{r^3} +$$

$$\frac{\pi^2 G^3 m_1 m_2^2 \left( \frac{3}{8} \vec{v}_1 \cdot \vec{v}_1 \hat{n} \times \vec{S}_1 \cdot \vec{v}_1 - \frac{15}{8} (\hat{n} \cdot \vec{v}_1)^2 \hat{n} \times \vec{S}_1 \cdot \vec{v}_1 \right)}{r^4} \Bigg\}$$

$$\left\{ \text{DiagSet}[3, 8, 32], \right.$$

$$, \emptyset \Bigg\}$$

$$\left\{ \text{DiagSet}[3, 8, 33], \right.$$

$$,$$

$$\frac{\pi^2 G^3 m_1 m_2^2 \left( -\frac{15}{8} (\hat{n} \cdot \vec{v}_2)^2 \hat{n} \times \vec{S}_1 \cdot \vec{v}_1 + \frac{3}{4} \hat{n} \cdot \vec{v}_2 \vec{S}_1 \times \vec{v}_1 \cdot \vec{v}_2 + \frac{3}{8} \vec{v}_2 \cdot \vec{v}_2 \hat{n} \times \vec{S}_1 \cdot \vec{v}_1 \right)}{r^4} \Bigg\}$$

$$\left\{ \text{DiagSet}[3, 8, 34], \right.$$

$$,$$

$$\frac{1}{r^3} \pi^2 G^3 m_1 m_2^2 \left( -\frac{3}{8} \hat{n} \cdot \vec{v}_2 \hat{n} \times \vec{a}_1 \cdot \vec{S}_1 + \frac{1}{8} \vec{a}_1 \times \vec{S}_1 \cdot \vec{v}_2 + \frac{3}{8} \hat{n} \cdot \vec{v}_2 \hat{n} \times \vec{S}_1 \cdot \vec{v}_1 - \frac{1}{8} \vec{S}_1 \times \vec{v}_1 \cdot \vec{v}_2 \right) +$$

$$\frac{1}{r^4} \pi^2 G^3 m_1 m_2^2 \left( -\frac{15}{8} (\hat{n} \cdot \vec{v}_2)^2 \hat{n} \times \vec{S}_1 \cdot \vec{v}_1 + \frac{3}{4} \hat{n} \cdot \vec{v}_2 \vec{S}_1 \times \vec{v}_1 \cdot \vec{v}_2 - \right.$$

$$\frac{15}{8} \hat{n} \cdot \vec{v}_1 \hat{n} \cdot \vec{v}_2 \hat{n} \times \vec{S}_1 \cdot \vec{v}_1 + \frac{3}{8} \hat{n} \cdot \vec{v}_1 \vec{S}_1 \times \vec{v}_1 \cdot \vec{v}_2 + \frac{3}{8} \vec{v}_1 \cdot \vec{v}_2 \hat{n} \times \vec{S}_1 \cdot \vec{v}_1 + \frac{3}{8} \vec{v}_2 \cdot \vec{v}_2 \hat{n} \times \vec{S}_1 \cdot \vec{v}_1 \Bigg\}$$

{DiagSet[3, 8, 35], 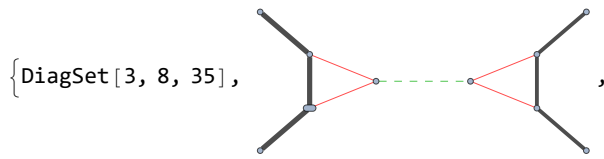 ,

$$\frac{1}{r^3} \pi^2 G^3 m_1 m_2^2 \left( -\frac{9}{32} \hat{n} \cdot \vec{v}_2 \hat{n} \times \vec{S}_1 \cdot \vec{a}_1 + \frac{3}{32} \vec{S}_1 \times \vec{a}_1 \cdot \vec{v}_2 - \frac{9}{32} \hat{n} \cdot \vec{v}_2 \hat{n} \times \vec{S}_1 \cdot \vec{v}_1 + \frac{3}{32} \vec{S}_1 \times \vec{v}_1 \cdot \vec{v}_2 \right) +$$

$$\frac{1}{r^4} \pi^2 G^3 m_1 m_2^2 \left( -\frac{9}{32} \hat{n} \cdot \vec{v}_1 \vec{S}_1 \times \vec{v}_1 \cdot \vec{v}_2 + \frac{45}{32} \hat{n} \cdot \vec{v}_2 \hat{n} \cdot \vec{v}_1 \hat{n} \times \vec{S}_1 \cdot \vec{v}_1 - \frac{9}{32} \vec{v}_1 \cdot \vec{v}_2 \hat{n} \times \vec{S}_1 \cdot \vec{v}_1 \right) \Bigg\}$$

{DiagSet[3, 8, 36], 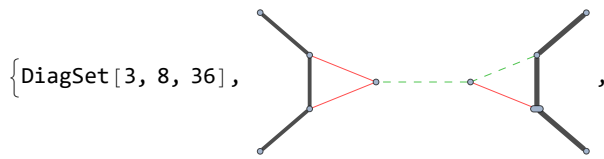 ,

$$\frac{\pi^2 G^3 m_1 m_2^2 \left( \frac{3}{8} \hat{n} \cdot \vec{v}_1 \vec{S}_1 \times \vec{v}_1 \cdot \vec{v}_2 - \frac{15}{8} \hat{n} \cdot \vec{v}_2 \hat{n} \cdot \vec{v}_1 \hat{n} \times \vec{S}_1 \cdot \vec{v}_1 + \frac{3}{8} \vec{v}_1 \cdot \vec{v}_2 \hat{n} \times \vec{S}_1 \cdot \vec{v}_1 \right)}{r^4} \Bigg\}$$

{DiagSet[3, 8, 37], 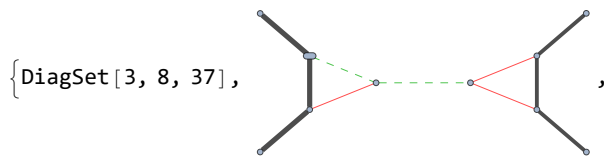 ,

$$\frac{1}{r^3} \pi^2 G^3 m_1 m_2^2 \left( -\frac{3}{4} \hat{n} \cdot \vec{v}_2 \hat{n} \times \vec{a}_1 \cdot \vec{S}_1 + \frac{1}{4} \vec{a}_1 \times \vec{S}_1 \cdot \vec{v}_2 + \frac{3}{4} \hat{n} \cdot \vec{v}_2 \hat{n} \times \vec{S}_1 \cdot \vec{v}_1 - \frac{1}{4} \vec{S}_1 \times \vec{v}_1 \cdot \vec{v}_2 \right) +$$

$$\frac{1}{r^4} \pi^2 G^3 m_1 m_2^2 \left( \frac{9}{16} \hat{n} \cdot \vec{v}_1 \vec{S}_1 \times \vec{v}_1 \cdot \vec{v}_2 - \frac{45}{16} \hat{n} \cdot \vec{v}_2 \hat{n} \cdot \vec{v}_1 \hat{n} \times \vec{S}_1 \cdot \vec{v}_1 + \frac{9}{16} \vec{v}_1 \cdot \vec{v}_2 \hat{n} \times \vec{S}_1 \cdot \vec{v}_1 \right) \Bigg\}$$

{DiagSet[3, 8, 38], 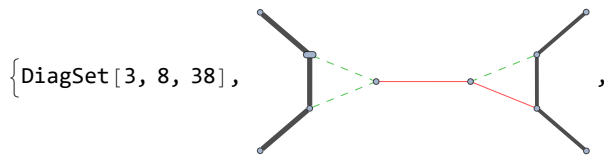 ,

$$\frac{\pi^2 G^3 m_1 m_2^2 \left( \frac{3}{2} \hat{n} \cdot \vec{v}_2 \hat{n} \times \vec{a}_1 \cdot \vec{S}_1 - \frac{1}{2} \vec{a}_1 \times \vec{S}_1 \cdot \vec{v}_2 - \frac{3}{2} \hat{n} \cdot \vec{v}_2 \hat{n} \times \vec{S}_1 \cdot \vec{v}_1 + \frac{1}{2} \vec{S}_1 \times \vec{v}_1 \cdot \vec{v}_2 \right)}{r^3} +$$

$$\frac{1}{r^4} \pi^2 G^3 m_1 m_2^2 \left( \frac{15}{2} (\hat{n} \cdot \vec{v}_2)^2 \hat{n} \times \vec{S}_1 \cdot \vec{v}_1 - 3 \hat{n} \cdot \vec{v}_2 \vec{S}_1 \times \vec{v}_1 \cdot \vec{v}_2 + \right.$$

$$\left. \frac{15}{2} \hat{n} \cdot \vec{v}_1 \hat{n} \cdot \vec{v}_2 \hat{n} \times \vec{S}_1 \cdot \vec{v}_1 - \frac{3}{2} \hat{n} \cdot \vec{v}_1 \vec{S}_1 \times \vec{v}_1 \cdot \vec{v}_2 - \frac{3}{2} \vec{v}_1 \cdot \vec{v}_2 \hat{n} \times \vec{S}_1 \cdot \vec{v}_1 - \frac{3}{2} \vec{v}_2 \cdot \vec{v}_2 \hat{n} \times \vec{S}_1 \cdot \vec{v}_1 \right) \Bigg\}$$

{DiagSet[3, 8, 39], 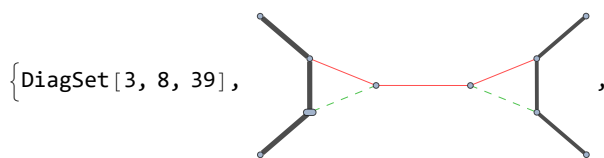 ,

$$\frac{1}{r^3} \pi^2 G^3 m_1 m_2^2 \left( -\frac{3}{8} \hat{n} \cdot \vec{v}_2 \hat{n} \times \vec{S}_1 \cdot \vec{a}_1 + \frac{1}{8} \vec{S}_1 \times \vec{a}_1 \cdot \vec{v}_2 - \frac{3}{8} \hat{n} \cdot \vec{v}_2 \hat{n} \times \vec{S}_1 \cdot \vec{v}_1 + \frac{1}{8} \vec{S}_1 \times \vec{v}_1 \cdot \vec{v}_2 \right) +$$

$$\frac{1}{r^4} \pi^2 G^3 m_1 m_2^2 \left( \frac{15}{8} (\hat{n} \cdot \vec{v}_2)^2 \hat{n} \times \vec{S}_1 \cdot \vec{v}_1 - \frac{3}{4} \hat{n} \cdot \vec{v}_2 \vec{S}_1 \times \vec{v}_1 \cdot \vec{v}_2 + \right.$$

$$\frac{15}{8} \hat{n} \cdot \vec{v}_1 \hat{n} \cdot \vec{v}_2 \hat{n} \times \vec{S}_1 \cdot \vec{v}_1 - \frac{3}{8} \hat{n} \cdot \vec{v}_1 \vec{S}_1 \times \vec{v}_1 \cdot \vec{v}_2 - \frac{3}{8} \vec{v}_1 \cdot \vec{v}_2 \hat{n} \times \vec{S}_1 \cdot \vec{v}_1 - \frac{3}{8} \vec{v}_2 \cdot \vec{v}_2 \hat{n} \times \vec{S}_1 \cdot \vec{v}_1 \Bigg\}$$

$$\left\{ \text{DiagSet}[3, 8, 40], \right. , \left. 0 \right\}$$
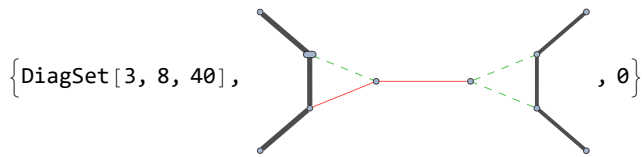

$$\left\{ \text{DiagSet}[3, 8, 41], \right. ,$$
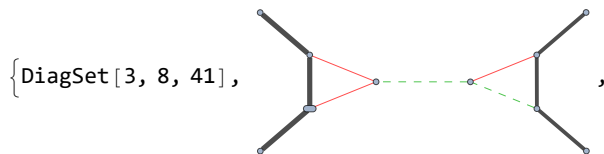

$$\frac{\pi^2 G^3 m_1 m_2^2 \left( \frac{3}{2} \hat{n} \cdot \vec{v}_2 \hat{n} \times \vec{S}_1 \cdot \vec{a}_1 - \frac{1}{2} \vec{S}_1 \times \vec{a}_1 \cdot \vec{v}_2 + \frac{3}{2} \hat{n} \cdot \vec{v}_2 \hat{n} \times \vec{S}_1 \cdot \vec{v}_1 - \frac{1}{2} \vec{S}_1 \times \vec{v}_1 \cdot \vec{v}_2 \right)}{r^3} +$$

$$\frac{1}{r^4} \pi^2 G^3 m_1 m_2^2 \left( \frac{3}{2} \hat{n} \cdot \vec{v}_1 \vec{S}_1 \times \vec{v}_1 \cdot \vec{v}_2 - \frac{15}{2} \hat{n} \cdot \vec{v}_2 \hat{n} \cdot \vec{v}_1 \hat{n} \times \vec{S}_1 \cdot \vec{v}_1 + \frac{3}{2} \vec{v}_1 \cdot \vec{v}_2 \hat{n} \times \vec{S}_1 \cdot \vec{v}_1 \right) \Bigg\}$$

$$\left\{ \text{DiagSet}[3, 8, 42], \right. , \left. \frac{1}{r^4} \right\}$$
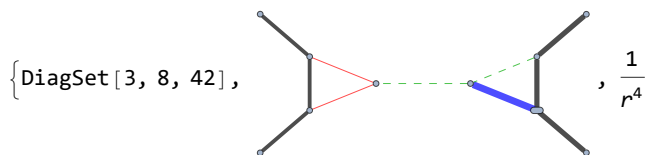

$$\pi^2 G^3 m_1 m_2^2 \left( -\frac{9}{32} \hat{n} \cdot \vec{v}_1 \vec{S}_1 \times \vec{v}_1 \cdot \vec{v}_2 + \frac{45}{32} \hat{n} \cdot \vec{v}_2 \hat{n} \cdot \vec{v}_1 \hat{n} \times \vec{S}_1 \cdot \vec{v}_1 - \frac{9}{32} \vec{v}_1 \cdot \vec{v}_2 \hat{n} \times \vec{S}_1 \cdot \vec{v}_1 \right) \Bigg\}$$

$$\left\{ \text{DiagSet}[3, 8, 43], \right. , \left. \frac{1}{r^4} \right\}$$
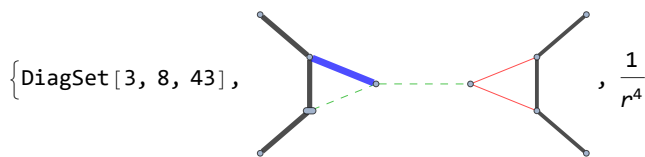

$$\pi^2 G^3 m_1 m_2^2 \left( -\frac{45}{32} (\hat{n} \cdot \vec{v}_1)^2 \hat{n} \times \vec{S}_1 \cdot \vec{v}_2 - \frac{9}{32} \hat{n} \cdot \vec{v}_1 \vec{S}_1 \times \vec{v}_1 \cdot \vec{v}_2 - \frac{45}{32} \hat{n} \cdot \vec{v}_2 \hat{n} \cdot \vec{v}_1 \hat{n} \times \vec{S}_1 \cdot \vec{v}_1 + \right. \\ \left. \frac{9}{32} \vec{v}_1 \cdot \vec{v}_1 \hat{n} \times \vec{S}_1 \cdot \vec{v}_2 + \frac{9}{32} \vec{v}_1 \cdot \vec{v}_2 \hat{n} \times \vec{S}_1 \cdot \vec{v}_1 \right) \Bigg\}$$

$$\left\{ \text{DiagSet}[3, 8, 44], \right. ,$$
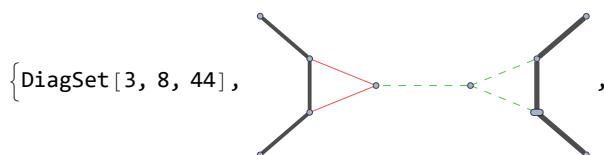

$$\frac{1}{r^3} \pi^2 G^3 m_1 m_2^2 \left( \frac{3}{32} \hat{n} \cdot \vec{a}_2 \hat{n} \times \vec{S}_1 \cdot \vec{v}_1 + \frac{9}{32} \hat{n} \cdot \vec{v}_1 \hat{n} \times \vec{S}_1 \cdot \vec{a}_2 + \frac{15}{32} \hat{n} \cdot \vec{v}_2 \hat{n} \times \vec{S}_1 \cdot \vec{a}_1 - \right. \\ \left. \frac{5}{32} \vec{S}_1 \times \vec{a}_1 \cdot \vec{v}_2 + \frac{1}{16} \vec{S}_1 \times \vec{v}_1 \cdot \vec{a}_2 - \frac{3}{8} \hat{n} \cdot \vec{v}_1 \hat{n} \times \vec{S}_1 \cdot \vec{v}_2 + \frac{9}{32} \hat{n} \cdot \vec{v}_2 \hat{n} \times \vec{S}_1 \cdot \vec{v}_1 - \frac{7}{32} \vec{S}_1 \times \vec{v}_1 \cdot \vec{v}_2 \right) + \\ \frac{1}{r^4} \pi^2 G^3 m_1 m_2^2 \left( \frac{45}{32} (\hat{n} \cdot \vec{v}_1)^2 \hat{n} \times \vec{S}_1 \cdot \vec{v}_2 + \frac{27}{32} \hat{n} \cdot \vec{v}_1 \vec{S}_1 \times \vec{v}_1 \cdot \vec{v}_2 - \frac{45}{32} \hat{n} \cdot \vec{v}_2 \hat{n} \cdot \vec{v}_1 \hat{n} \times \vec{S}_1 \cdot \vec{v}_1 + \right. \\ \left. \frac{45}{32} \hat{n} \cdot \vec{v}_2 \hat{n} \cdot \vec{v}_1 \hat{n} \times \vec{S}_1 \cdot \vec{v}_2 + \frac{15}{32} (\hat{n} \cdot \vec{v}_2)^2 \hat{n} \times \vec{S}_1 \cdot \vec{v}_1 + \frac{3}{32} \hat{n} \cdot \vec{v}_2 \vec{S}_1 \times \vec{v}_1 \cdot \vec{v}_2 - \right. \\ \left. \frac{9}{32} \vec{v}_1 \cdot \vec{v}_1 \hat{n} \times \vec{S}_1 \cdot \vec{v}_2 + \frac{9}{32} \vec{v}_1 \cdot \vec{v}_2 \hat{n} \times \vec{S}_1 \cdot \vec{v}_1 - \frac{9}{32} \vec{v}_1 \cdot \vec{v}_2 \hat{n} \times \vec{S}_1 \cdot \vec{v}_2 - \frac{3}{32} \vec{v}_2 \cdot \vec{v}_2 \hat{n} \times \vec{S}_1 \cdot \vec{v}_1 \right) \Bigg\}$$



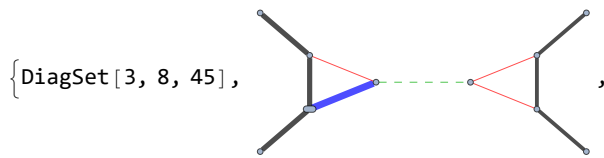

$$\frac{\pi^2 G^3 m_1 m_2^2 \left( \frac{3}{32} \hat{n} \cdot \vec{a}_2 \hat{n} \times \vec{S}_1 \cdot \vec{v}_1 - \frac{3}{32} \hat{n} \cdot \vec{v}_1 \hat{n} \times \vec{S}_1 \cdot \vec{a}_2 - \frac{1}{16} \vec{S}_1 \times \vec{v}_1 \cdot \vec{a}_2 \right)}{r^3} + \frac{1}{r^4}$$

$$\pi^2 G^3 m_1 m_2^2 \left( \frac{15}{32} (\hat{n} \cdot \vec{v}_1)^2 \hat{n} \times \vec{S}_1 \cdot \vec{v}_2 + \frac{3}{8} \hat{n} \cdot \vec{v}_1 \vec{S}_1 \times \vec{v}_1 \cdot \vec{v}_2 - \frac{15}{16} \hat{n} \cdot \vec{v}_2 \hat{n} \cdot \vec{v}_1 \hat{n} \times \vec{S}_1 \cdot \vec{v}_1 - \right.$$

$$\frac{15}{32} \hat{n} \cdot \vec{v}_2 \hat{n} \cdot \vec{v}_1 \hat{n} \times \vec{S}_1 \cdot \vec{v}_2 + \frac{15}{32} (\hat{n} \cdot \vec{v}_2)^2 \hat{n} \times \vec{S}_1 \cdot \vec{v}_1 - \frac{9}{32} \hat{n} \cdot \vec{v}_2 \vec{S}_1 \times \vec{v}_1 \cdot \vec{v}_2 -$$

$$\left. \frac{3}{32} \vec{v}_1 \cdot \vec{v}_1 \hat{n} \times \vec{S}_1 \cdot \vec{v}_2 + \frac{3}{16} \vec{v}_1 \cdot \vec{v}_2 \hat{n} \times \vec{S}_1 \cdot \vec{v}_1 + \frac{3}{32} \vec{v}_1 \cdot \vec{v}_2 \hat{n} \times \vec{S}_1 \cdot \vec{v}_2 - \frac{3}{32} \vec{v}_2 \cdot \vec{v}_2 \hat{n} \times \vec{S}_1 \cdot \vec{v}_1 \right)$$

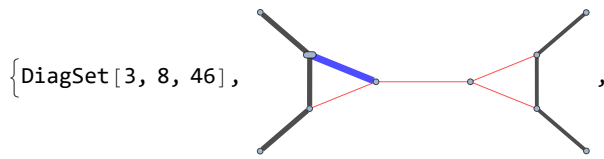

$$\frac{\pi^2 G^3 m_1 m_2^2 \left( \frac{3}{8} \hat{n} \cdot \vec{v}_2 \hat{n} \times \vec{a}_1 \cdot \vec{S}_1 - \frac{1}{8} \vec{a}_1 \times \vec{S}_1 \cdot \vec{v}_2 - \frac{3}{8} \hat{n} \cdot \vec{v}_2 \hat{n} \times \vec{S}_1 \cdot \vec{v}_1 + \frac{1}{8} \vec{S}_1 \times \vec{v}_1 \cdot \vec{v}_2 \right)}{r^3} +$$

$$\frac{1}{r^4} \pi^2 G^3 m_1 m_2^2 \left( -\frac{15}{64} (\hat{n} \cdot \vec{v}_2)^2 \hat{n} \times \vec{S}_1 \cdot \vec{v}_1 + \frac{3}{32} \hat{n} \cdot \vec{v}_2 \vec{S}_1 \times \vec{v}_1 \cdot \vec{v}_2 + \right.$$

$$\left. \frac{15}{8} \hat{n} \cdot \vec{v}_1 \hat{n} \cdot \vec{v}_2 \hat{n} \times \vec{S}_1 \cdot \vec{v}_1 - \frac{3}{8} \hat{n} \cdot \vec{v}_1 \vec{S}_1 \times \vec{v}_1 \cdot \vec{v}_2 - \frac{3}{8} \vec{v}_1 \cdot \vec{v}_2 \hat{n} \times \vec{S}_1 \cdot \vec{v}_1 + \frac{3}{64} \vec{v}_2 \cdot \vec{v}_2 \hat{n} \times \vec{S}_1 \cdot \vec{v}_1 \right)$$

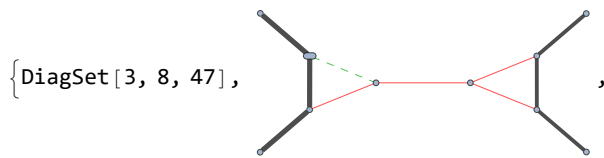

$$\frac{1}{r^3} \pi^2 G^3 m_1 m_2^2 \left( -\frac{3}{8} \hat{n} \cdot \vec{v}_2 \hat{n} \times \vec{a}_1 \cdot \vec{S}_1 + \frac{1}{8} \vec{a}_1 \times \vec{S}_1 \cdot \vec{v}_2 + \frac{3}{8} \hat{n} \cdot \vec{v}_2 \hat{n} \times \vec{S}_1 \cdot \vec{v}_1 - \frac{1}{8} \vec{S}_1 \times \vec{v}_1 \cdot \vec{v}_2 \right) +$$

$$\frac{1}{r^4} \pi^2 G^3 m_1 m_2^2 \left( \frac{15}{64} (\hat{n} \cdot \vec{v}_2)^2 \hat{n} \times \vec{S}_1 \cdot \vec{v}_1 - \frac{3}{32} \hat{n} \cdot \vec{v}_2 \vec{S}_1 \times \vec{v}_1 \cdot \vec{v}_2 - \right.$$

$$\left. \frac{15}{8} \hat{n} \cdot \vec{v}_1 \hat{n} \cdot \vec{v}_2 \hat{n} \times \vec{S}_1 \cdot \vec{v}_1 + \frac{3}{8} \hat{n} \cdot \vec{v}_1 \vec{S}_1 \times \vec{v}_1 \cdot \vec{v}_2 + \frac{3}{8} \vec{v}_1 \cdot \vec{v}_2 \hat{n} \times \vec{S}_1 \cdot \vec{v}_1 - \frac{3}{64} \vec{v}_2 \cdot \vec{v}_2 \hat{n} \times \vec{S}_1 \cdot \vec{v}_1 \right)$$

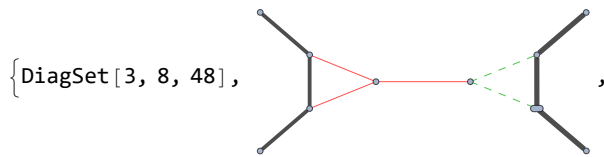

$$\frac{\pi^2 G^3 m_1 m_2^2 \left( \frac{3}{2} \hat{n} \cdot \vec{v}_2 \hat{n} \times \vec{S}_1 \cdot \vec{a}_1 - \frac{1}{2} \vec{S}_1 \times \vec{a}_1 \cdot \vec{v}_2 + \frac{3}{2} \hat{n} \cdot \vec{v}_2 \hat{n} \times \vec{S}_1 \cdot \vec{v}_1 - \frac{1}{2} \vec{S}_1 \times \vec{v}_1 \cdot \vec{v}_2 \right)}{r^3} +$$

$$\frac{1}{r^4} \pi^2 G^3 m_1 m_2^2 \left( \frac{15}{16} (\hat{n} \cdot \vec{v}_2)^2 \hat{n} \times \vec{S}_1 \cdot \vec{v}_1 - \frac{3}{8} \hat{n} \cdot \vec{v}_2 \vec{S}_1 \times \vec{v}_1 \cdot \vec{v}_2 - \right.$$

$$\left. \frac{15}{2} \hat{n} \cdot \vec{v}_1 \hat{n} \cdot \vec{v}_2 \hat{n} \times \vec{S}_1 \cdot \vec{v}_1 + \frac{3}{2} \hat{n} \cdot \vec{v}_1 \vec{S}_1 \times \vec{v}_1 \cdot \vec{v}_2 + \frac{3}{2} \vec{v}_1 \cdot \vec{v}_2 \hat{n} \times \vec{S}_1 \cdot \vec{v}_1 - \frac{3}{16} \vec{v}_2 \cdot \vec{v}_2 \hat{n} \times \vec{S}_1 \cdot \vec{v}_1 \right)$$

{DiagSet[3, 8, 49],

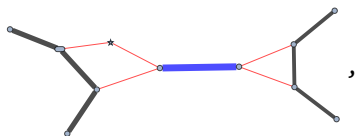

,

$$\frac{1}{r^3} \pi^2 G^3 m_1 m_2^2 \left( \frac{3}{32} \hat{n} \cdot \vec{v}_2 \hat{n} \times \vec{S}_1 \cdot \vec{a}_1 - \frac{1}{32} \vec{S}_1 \times \vec{a}_1 \cdot \vec{v}_2 + \frac{3}{32} \hat{n} \cdot \vec{v}_2 \hat{n} \times \vec{S}_1 \cdot \vec{v}_1 - \frac{1}{32} \vec{S}_1 \times \vec{v}_1 \cdot \vec{v}_2 \right) +$$

$$\frac{1}{r^4} \pi^2 G^3 m_1 m_2^2 \left( \frac{15}{256} (\hat{n} \cdot \vec{v}_1)^2 \hat{n} \times \vec{S}_1 \cdot \vec{v}_1 + \frac{3}{32} \hat{n} \cdot \vec{v}_1 \vec{S}_1 \times \vec{v}_1 \cdot \vec{v}_2 - \right.$$

$$\left. \frac{15}{32} \hat{n} \cdot \vec{v}_2 \hat{n} \cdot \vec{v}_1 \hat{n} \times \vec{S}_1 \cdot \vec{v}_1 - \frac{3}{256} \vec{v}_1 \cdot \vec{v}_1 \hat{n} \times \vec{S}_1 \cdot \vec{v}_1 + \frac{3}{32} \vec{v}_1 \cdot \vec{v}_2 \hat{n} \times \vec{S}_1 \cdot \vec{v}_1 \right\}$$

{DiagSet[3, 8, 50],

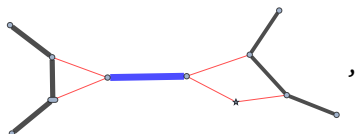

,

$$\frac{1}{r^3} \pi^2 G^3 m_1 m_2^2 \left( -\frac{3}{32} \hat{n} \cdot \vec{v}_2 \hat{n} \times \vec{a}_1 \cdot \vec{S}_1 + \frac{1}{32} \vec{a}_1 \times \vec{S}_1 \cdot \vec{v}_2 + \frac{3}{32} \hat{n} \cdot \vec{v}_2 \hat{n} \times \vec{S}_1 \cdot \vec{v}_1 - \frac{1}{32} \vec{S}_1 \times \vec{v}_1 \cdot \vec{v}_2 \right) +$$

$$\frac{1}{r^4} \pi^2 G^3 m_1 m_2^2 \left( \frac{3}{32} \hat{n} \cdot \vec{v}_1 \vec{S}_1 \times \vec{v}_1 \cdot \vec{v}_2 - \frac{15}{32} \hat{n} \cdot \vec{v}_2 \hat{n} \cdot \vec{v}_1 \hat{n} \times \vec{S}_1 \cdot \vec{v}_1 + \frac{3}{32} \vec{v}_1 \cdot \vec{v}_2 \hat{n} \times \vec{S}_1 \cdot \vec{v}_1 \right\}$$

{DiagSet[3, 8, 51],

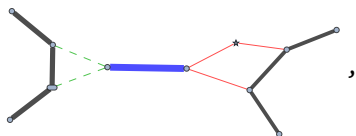

,

$$\frac{1}{r^3} \pi^2 G^3 m_1 m_2^2 \left( -\frac{3}{32} \hat{n} \cdot \vec{a}_1 \hat{n} \times \vec{S}_1 \cdot \vec{v}_2 - \frac{3}{32} \hat{n} \cdot \vec{v}_2 \hat{n} \times \vec{a}_1 \cdot \vec{S}_1 + \frac{1}{16} \vec{a}_1 \times \vec{S}_1 \cdot \vec{v}_2 - \right.$$

$$\left. \frac{3}{32} \hat{n} \cdot \vec{v}_1 \hat{n} \times \vec{S}_1 \cdot \vec{v}_2 + \frac{3}{32} \hat{n} \cdot \vec{v}_2 \hat{n} \times \vec{S}_1 \cdot \vec{v}_1 - \frac{1}{16} \vec{S}_1 \times \vec{v}_1 \cdot \vec{v}_2 \right) + \frac{1}{r^4}$$

$$\pi^2 G^3 m_1 m_2^2 \left( \frac{15}{32} (\hat{n} \cdot \vec{v}_1)^2 \hat{n} \times \vec{S}_1 \cdot \vec{v}_2 + \frac{9}{32} \hat{n} \cdot \vec{v}_1 \vec{S}_1 \times \vec{v}_1 \cdot \vec{v}_2 - \frac{15}{32} \hat{n} \cdot \vec{v}_2 \hat{n} \cdot \vec{v}_1 \hat{n} \times \vec{S}_1 \cdot \vec{v}_1 - \frac{15}{32} \hat{n} \cdot \vec{v}_2 \hat{n} \cdot \vec{v}_1 \hat{n} \times \vec{S}_1 \cdot \vec{v}_2 + \right.$$

$$\left. \frac{15}{32} (\hat{n} \cdot \vec{v}_2)^2 \hat{n} \times \vec{S}_1 \cdot \vec{v}_1 - \frac{9}{32} \hat{n} \cdot \vec{v}_2 \vec{S}_1 \times \vec{v}_1 \cdot \vec{v}_2 - \frac{3}{32} \vec{v}_1 \cdot \vec{v}_1 \hat{n} \times \vec{S}_1 \cdot \vec{v}_2 + \right.$$

$$\left. \frac{3}{32} \vec{v}_1 \cdot \vec{v}_2 \hat{n} \times \vec{S}_1 \cdot \vec{v}_1 + \frac{3}{32} \vec{v}_1 \cdot \vec{v}_2 \hat{n} \times \vec{S}_1 \cdot \vec{v}_2 - \frac{3}{32} \vec{v}_2 \cdot \vec{v}_2 \hat{n} \times \vec{S}_1 \cdot \vec{v}_1 \right\}$$

{DiagSet[3, 8, 52],

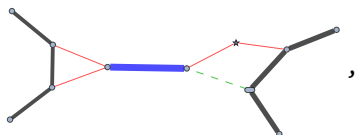

,

$$\frac{1}{r^3} \pi^2 G^3 m_1 m_2^2 \left( -\frac{3}{64} \hat{n} \cdot \vec{a}_1 \hat{n} \times \vec{S}_1 \cdot \vec{v}_1 + \frac{3}{64} \hat{n} \cdot \vec{v}_1 \hat{n} \times \vec{a}_1 \cdot \vec{S}_1 - \frac{9}{64} \hat{n} \cdot \vec{v}_2 \hat{n} \times \vec{a}_1 \cdot \vec{S}_1 + \right.$$

$$\left. \frac{3}{64} \vec{a}_1 \times \vec{S}_1 \cdot \vec{v}_2 - \frac{3}{16} \hat{n} \cdot \vec{v}_1 \hat{n} \times \vec{S}_1 \cdot \vec{v}_1 + \frac{9}{64} \hat{n} \cdot \vec{v}_2 \hat{n} \times \vec{S}_1 \cdot \vec{v}_1 - \frac{3}{64} \vec{S}_1 \times \vec{v}_1 \cdot \vec{v}_2 \right) +$$

$$\frac{\pi^2 G^3 m_1 m_2^2 \left( \frac{3}{64} \hat{n} \times \vec{S}_1 \cdot \vec{v}_1 - \frac{3}{64} \hat{n} \times \vec{a}_1 \cdot \vec{S}_1 \right)}{r^2} + \frac{1}{r^4} \pi^2 G^3 m_1 m_2^2 \left( \frac{15}{64} (\hat{n} \cdot \vec{v}_1)^2 \hat{n} \times \vec{S}_1 \cdot \vec{v}_1 + \frac{9}{64} \hat{n} \cdot \vec{v}_1 \vec{S}_1 \times \vec{v}_1 \cdot \vec{v}_2 - \right.$$

$$\left. \frac{45}{64} \hat{n} \cdot \vec{v}_2 \hat{n} \cdot \vec{v}_1 \hat{n} \times \vec{S}_1 \cdot \vec{v}_1 - \frac{3}{64} \vec{v}_1 \cdot \vec{v}_1 \hat{n} \times \vec{S}_1 \cdot \vec{v}_1 + \frac{9}{64} \vec{v}_1 \cdot \vec{v}_2 \hat{n} \times \vec{S}_1 \cdot \vec{v}_1 \right\}$$

$$\left\{ \text{DiagSet}[3, 8, 53], \right.$$
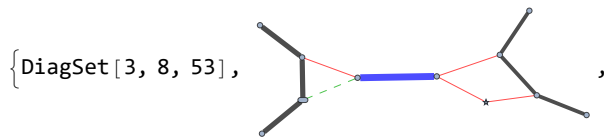

$$,$$

$$\frac{1}{r^3} \pi^2 G^3 m_1 m_2^2 \left( \frac{3}{32} \hat{n} \cdot \vec{v}_2 \hat{n} \times \vec{a}_1 \cdot \vec{S}_1 - \frac{1}{32} \vec{a}_1 \times \vec{S}_1 \cdot \vec{v}_2 - \frac{3}{32} \hat{n} \cdot \vec{v}_1 \hat{n} \times \vec{S}_1 \cdot \vec{v}_2 - \frac{3}{32} \hat{n} \cdot \vec{v}_2 \hat{n} \times \vec{S}_1 \cdot \vec{v}_1 \right) +$$

$$\frac{1}{r^4} \pi^2 G^3 m_1 m_2^2 \left( -\frac{15}{64} (\hat{n} \cdot \vec{v}_2)^2 \hat{n} \times \vec{S}_1 \cdot \vec{v}_1 + \frac{3}{32} \hat{n} \cdot \vec{v}_2 \vec{S}_1 \times \vec{v}_1 \cdot \vec{v}_2 + \frac{15}{32} \hat{n} \cdot \vec{v}_1 \hat{n} \cdot \vec{v}_2 \hat{n} \times \vec{S}_1 \cdot \vec{v}_1 - \right.$$

$$\left. \frac{3}{32} \hat{n} \cdot \vec{v}_1 \vec{S}_1 \times \vec{v}_1 \cdot \vec{v}_2 - \frac{3}{32} \vec{v}_1 \cdot \vec{v}_2 \hat{n} \times \vec{S}_1 \cdot \vec{v}_1 + \frac{3}{64} \vec{v}_2 \cdot \vec{v}_2 \hat{n} \times \vec{S}_1 \cdot \vec{v}_1 \right) + \frac{\pi^2 G^3 m_1 m_2^2 \hat{n} \times \vec{S}_1 \cdot \vec{v}_2}{32 r^2} \Big\}$$

$$\left\{ \text{DiagSet}[3, 8, 54], \right.$$
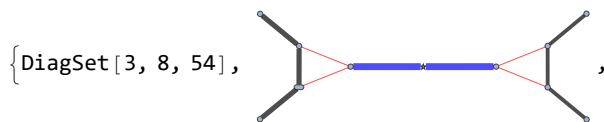

$$,$$

$$\frac{1}{r^3} \pi^2 G^3 m_1 m_2^2 \left( -\frac{3}{32} \hat{n} \cdot \vec{v}_2 \hat{n} \times \vec{S}_1 \cdot \vec{a}_1 + \frac{1}{32} \vec{S}_1 \times \vec{a}_1 \cdot \vec{v}_2 - \frac{3}{32} \hat{n} \cdot \vec{v}_2 \hat{n} \times \vec{S}_1 \cdot \vec{v}_1 + \frac{1}{32} \vec{S}_1 \times \vec{v}_1 \cdot \vec{v}_2 \right) +$$

$$\frac{1}{r^4} \pi^2 G^3 m_1 m_2^2 \left( -\frac{3}{32} \hat{n} \cdot \vec{v}_1 \vec{S}_1 \times \vec{v}_1 \cdot \vec{v}_2 + \frac{15}{32} \hat{n} \cdot \vec{v}_2 \hat{n} \cdot \vec{v}_1 \hat{n} \times \vec{S}_1 \cdot \vec{v}_1 - \frac{3}{32} \vec{v}_1 \cdot \vec{v}_2 \hat{n} \times \vec{S}_1 \cdot \vec{v}_1 \right) \Big\}$$

$$\left\{ \text{DiagSet}[3, 8, 55], \right.$$
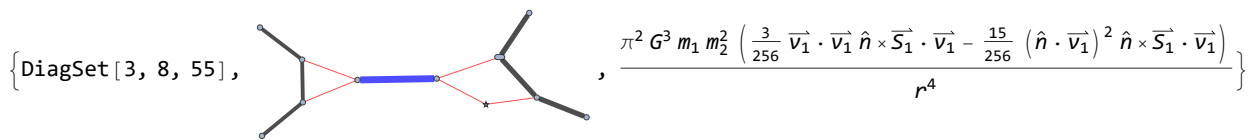

$$, \frac{\pi^2 G^3 m_1 m_2^2 \left( \frac{3}{256} \vec{v}_1 \cdot \vec{v}_1 \hat{n} \times \vec{S}_1 \cdot \vec{v}_1 - \frac{15}{256} (\hat{n} \cdot \vec{v}_1)^2 \hat{n} \times \vec{S}_1 \cdot \vec{v}_1 \right)}{r^4} \Big\}$$

$$\left\{ \text{DiagSet}[3, 8, 56], \right.$$
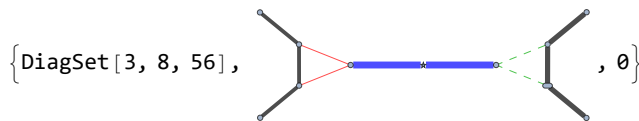

$$, \emptyset \Big\}$$

$$\left\{ \text{DiagSet}[3, 8, 57], \right.$$
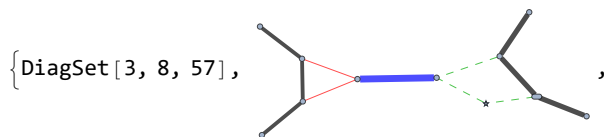

$$,$$

$$\frac{1}{r^3} \pi^2 G^3 m_1 m_2^2 \left( -\frac{3}{32} \hat{n} \cdot \vec{a}_1 \hat{n} \times \vec{S}_1 \cdot \vec{v}_1 - \frac{3}{32} \hat{n} \cdot \vec{v}_1 \hat{n} \times \vec{a}_1 \cdot \vec{S}_1 + \frac{1}{16} \vec{a}_1 \times \vec{S}_1 \cdot \vec{v}_1 + \frac{9}{32} \hat{n} \cdot \vec{v}_1 \hat{n} \times \vec{S}_1 \cdot \vec{v}_1 - \frac{9}{32} \hat{n} \cdot \vec{v}_2 \hat{n} \times \vec{S}_1 \cdot \vec{v}_1 + \right.$$

$$\left. \frac{3}{32} \vec{S}_1 \times \vec{v}_1 \cdot \vec{v}_2 \right) + \frac{3 \pi^2 G^3 m_1 m_2^2 \hat{n} \times \vec{a}_1 \cdot \vec{S}_1}{32 r^2} + \frac{\pi^2 G^3 m_1 m_2^2 \left( \frac{15}{256} (\hat{n} \cdot \vec{v}_1)^2 \hat{n} \times \vec{S}_1 \cdot \vec{v}_1 - \frac{3}{256} \vec{v}_1 \cdot \vec{v}_1 \hat{n} \times \vec{S}_1 \cdot \vec{v}_1 \right)}{r^4} \Big\}$$

$$\left\{ \text{DiagSet}[3, 8, 58], \right.$$
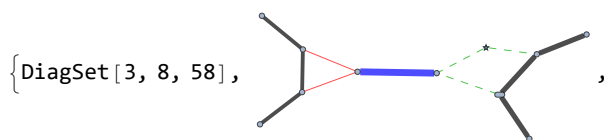

$$,$$

$$\frac{\pi^2 G^3 m_1 m_2^2 \left( \frac{3}{32} \hat{n} \cdot \vec{v}_2 \hat{n} \times \vec{a}_1 \cdot \vec{S}_1 - \frac{1}{32} \vec{a}_1 \times \vec{S}_1 \cdot \vec{v}_2 + \frac{3}{32} \hat{n} \cdot \vec{v}_1 \hat{n} \times \vec{S}_1 \cdot \vec{v}_1 \right)}{r^3} +$$

$$\frac{\pi^2 G^3 m_1 m_2^2 \hat{n} \times \vec{a}_1 \cdot \vec{S}_1}{32 r^2} + \frac{1}{r^4} \pi^2 G^3 m_1 m_2^2 \left( -\frac{15}{256} (\hat{n} \cdot \vec{v}_1)^2 \hat{n} \times \vec{S}_1 \cdot \vec{v}_1 - \frac{3}{32} \hat{n} \cdot \vec{v}_1 \vec{S}_1 \times \vec{v}_1 \cdot \vec{v}_2 + \right.$$

$$\left. \frac{15}{32} \hat{n} \cdot \vec{v}_2 \hat{n} \cdot \vec{v}_1 \hat{n} \times \vec{S}_1 \cdot \vec{v}_1 + \frac{3}{256} \vec{v}_1 \cdot \vec{v}_1 \hat{n} \times \vec{S}_1 \cdot \vec{v}_1 - \frac{3}{32} \vec{v}_1 \cdot \vec{v}_2 \hat{n} \times \vec{S}_1 \cdot \vec{v}_1 \right) \Big\}$$

$$\left\{ \text{DiagSet}[3, 8, 59], \right\}$$

$$\left\{ \text{DiagSet}[3, 8, 60], \right\}$$

$$\begin{aligned} & \frac{1}{r^3} \pi^2 G^3 m_1 m_2^2 \left( \frac{3}{64} \hat{n} \cdot \vec{a}_1 \hat{n} \times \vec{S}_1 \cdot \vec{v}_1 - \frac{3}{64} \hat{n} \cdot \vec{v}_1 \hat{n} \times \vec{a}_1 \cdot \vec{S}_1 + \frac{3}{64} \hat{n} \cdot \vec{v}_2 \hat{n} \times \vec{a}_1 \cdot \vec{S}_1 - \right. \\ & \left. \frac{1}{64} \vec{a}_1 \times \vec{S}_1 \cdot \vec{v}_2 - \frac{3}{64} \hat{n} \cdot \vec{v}_2 \hat{n} \times \vec{S}_1 \cdot \vec{v}_1 + \frac{1}{64} \vec{S}_1 \times \vec{v}_1 \cdot \vec{v}_2 \right) + \\ & \frac{\pi^2 G^3 m_1 m_2^2 \left( \frac{1}{64} \hat{n} \times \vec{S}_1 \cdot \vec{v}_1 - \frac{1}{64} \hat{n} \times \vec{a}_1 \cdot \vec{S}_1 \right)}{r^2} + \frac{1}{r^4} \pi^2 G^3 m_1 m_2^2 \left( -\frac{15}{64} (\hat{n} \cdot \vec{v}_1)^2 \hat{n} \times \vec{S}_1 \cdot \vec{v}_1 - \frac{3}{64} \hat{n} \cdot \vec{v}_1 \vec{S}_1 \times \vec{v}_1 \cdot \vec{v}_2 + \right. \\ & \left. \frac{15}{64} \hat{n} \cdot \vec{v}_2 \hat{n} \cdot \vec{v}_1 \hat{n} \times \vec{S}_1 \cdot \vec{v}_1 + \frac{3}{64} \vec{v}_1 \cdot \vec{v}_1 \hat{n} \times \vec{S}_1 \cdot \vec{v}_1 - \frac{3}{64} \vec{v}_1 \cdot \vec{v}_2 \hat{n} \times \vec{S}_1 \cdot \vec{v}_1 \right) \} \end{aligned}$$

$$\left\{ \text{DiagSet}[3, 8, 61], \right\}$$

$$\begin{aligned} & \frac{1}{r^3} \pi^2 G^3 m_1 m_2^2 \left( \frac{9}{64} \hat{n} \cdot \vec{a}_2 \hat{n} \times \vec{S}_1 \cdot \vec{v}_1 + \frac{3}{32} \hat{n} \cdot \vec{v}_1 \hat{n} \times \vec{a}_2 \cdot \vec{S}_1 - \frac{5}{64} \vec{a}_2 \times \vec{S}_1 \cdot \vec{v}_1 - \right. \\ & \left. \frac{3}{32} \hat{n} \cdot \vec{v}_1 \hat{n} \times \vec{S}_1 \cdot \vec{v}_2 + \frac{9}{64} \hat{n} \cdot \vec{v}_2 \hat{n} \times \vec{S}_1 \cdot \vec{v}_1 - \frac{5}{64} \vec{S}_1 \times \vec{v}_1 \cdot \vec{v}_2 \right) + \frac{1}{r^4} \\ & \pi^2 G^3 m_1 m_2^2 \left( \frac{45}{128} (\hat{n} \cdot \vec{v}_1)^2 \hat{n} \times \vec{S}_1 \cdot \vec{v}_2 + \frac{15}{64} \hat{n} \cdot \vec{v}_1 \vec{S}_1 \times \vec{v}_1 \cdot \vec{v}_2 - \frac{15}{32} \hat{n} \cdot \vec{v}_2 \hat{n} \cdot \vec{v}_1 \hat{n} \times \vec{S}_1 \cdot \vec{v}_1 - \frac{15}{32} \hat{n} \cdot \vec{v}_2 \hat{n} \cdot \vec{v}_1 \hat{n} \times \vec{S}_1 \cdot \vec{v}_2 + \right. \\ & \left. \frac{45}{64} (\hat{n} \cdot \vec{v}_2)^2 \hat{n} \times \vec{S}_1 \cdot \vec{v}_1 - \frac{3}{8} \hat{n} \cdot \vec{v}_2 \vec{S}_1 \times \vec{v}_1 \cdot \vec{v}_2 - \frac{9}{128} \vec{v}_1 \cdot \vec{v}_1 \hat{n} \times \vec{S}_1 \cdot \vec{v}_2 + \right. \\ & \left. \frac{3}{32} \vec{v}_1 \cdot \vec{v}_2 \hat{n} \times \vec{S}_1 \cdot \vec{v}_1 + \frac{3}{32} \vec{v}_1 \cdot \vec{v}_2 \hat{n} \times \vec{S}_1 \cdot \vec{v}_2 - \frac{9}{64} \vec{v}_2 \cdot \vec{v}_2 \hat{n} \times \vec{S}_1 \cdot \vec{v}_1 \right) \} \end{aligned}$$

$$\left\{ \text{DiagSet}[3, 8, 62], \right\}$$

$$\begin{aligned} & \frac{1}{r^3} \pi^2 G^3 m_1 m_2^2 \left( \frac{3}{16} \hat{n} \cdot \vec{a}_2 \hat{n} \times \vec{S}_1 \cdot \vec{v}_2 - \frac{3}{16} \hat{n} \cdot \vec{v}_1 \hat{n} \times \vec{a}_2 \cdot \vec{S}_1 + \frac{3}{16} \hat{n} \cdot \vec{v}_2 \hat{n} \times \vec{a}_2 \cdot \vec{S}_1 + \frac{1}{16} \vec{a}_2 \times \vec{S}_1 \cdot \vec{v}_1 - \frac{1}{8} \vec{a}_2 \times \vec{S}_1 \cdot \vec{v}_2 \right) + \\ & \frac{\pi^2 G^3 m_1 m_2^2 \hat{n} \times \vec{a}_2 \cdot \vec{S}_1}{16 r^2} + \frac{\pi^2 G^3 m_1 m_2^2 \left( \frac{15}{64} (\hat{n} \cdot \vec{v}_2)^2 \hat{n} \times \vec{S}_1 \cdot \vec{v}_2 - \frac{3}{64} \vec{v}_2 \cdot \vec{v}_2 \hat{n} \times \vec{S}_1 \cdot \vec{v}_2 \right)}{r^4} \} \end{aligned}$$

$$\left\{ \text{DiagSet}[3, 8, 63], \right\}$$

$$\begin{aligned} & \frac{\pi^2 G^3 m_1 m_2^2 \left( \frac{3}{32} \hat{n} \cdot \vec{v}_1 \hat{n} \times \vec{a}_2 \cdot \vec{S}_1 - \frac{1}{32} \vec{a}_2 \times \vec{S}_1 \cdot \vec{v}_1 + \frac{3}{32} \hat{n} \cdot \vec{v}_2 \hat{n} \times \vec{S}_1 \cdot \vec{v}_2 \right)}{r^3} - \frac{\pi^2 G^3 m_1 m_2^2 \hat{n} \times \vec{a}_2 \cdot \vec{S}_1}{32 r^2} + \\ & \frac{1}{r^4} \pi^2 G^3 m_1 m_2^2 \left( -\frac{3}{32} \hat{n} \cdot \vec{v}_2 \vec{S}_1 \times \vec{v}_1 \cdot \vec{v}_2 - \frac{15}{32} \hat{n} \cdot \vec{v}_1 \hat{n} \cdot \vec{v}_2 \hat{n} \times \vec{S}_1 \cdot \vec{v}_2 + \frac{3}{32} \vec{v}_1 \cdot \vec{v}_2 \hat{n} \times \vec{S}_1 \cdot \vec{v}_2 \right) \} \end{aligned}$$

{DiagSet[3, 8, 64], 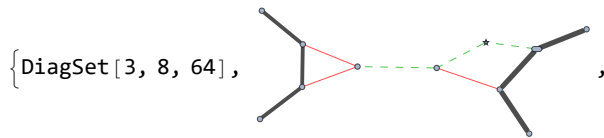,

$$\frac{1}{r^3} \pi^2 G^3 m_1 m_2^2 \left( -\frac{3}{64} \hat{n} \cdot \vec{a}_2 \hat{n} \times \vec{S}_1 \cdot \vec{v}_1 + \frac{9}{32} \hat{n} \cdot \vec{v}_1 \hat{n} \times \vec{a}_2 \cdot \vec{S}_1 - \frac{5}{64} \vec{a}_2 \times \vec{S}_1 \cdot \vec{v}_1 - \frac{9}{32} \hat{n} \cdot \vec{v}_1 \hat{n} \times \vec{S}_1 \cdot \vec{v}_2 + \right. \\ \left. \frac{3}{64} \hat{n} \cdot \vec{v}_2 \hat{n} \times \vec{S}_1 \cdot \vec{v}_1 + \frac{9}{16} \hat{n} \cdot \vec{v}_2 \hat{n} \times \vec{S}_1 \cdot \vec{v}_2 - \frac{7}{64} \vec{S}_1 \times \vec{v}_1 \cdot \vec{v}_2 \right) - \frac{3 \pi^2 G^3 m_1 m_2^2 \hat{n} \times \vec{a}_2 \cdot \vec{S}_1}{16 r^2} + \frac{1}{r^4} \\ \pi^2 G^3 m_1 m_2^2 \left( \frac{45}{128} (\hat{n} \cdot \vec{v}_1)^2 \hat{n} \times \vec{S}_1 \cdot \vec{v}_2 + \frac{9}{64} \hat{n} \cdot \vec{v}_1 \vec{S}_1 \times \vec{v}_1 \cdot \vec{v}_2 - \frac{45}{32} \hat{n} \cdot \vec{v}_2 \hat{n} \cdot \vec{v}_1 \hat{n} \times \vec{S}_1 \cdot \vec{v}_2 - \frac{15}{64} (\hat{n} \cdot \vec{v}_2)^2 \hat{n} \times \vec{S}_1 \cdot \vec{v}_1 - \right. \\ \left. \frac{3}{16} \hat{n} \cdot \vec{v}_2 \vec{S}_1 \times \vec{v}_1 \cdot \vec{v}_2 - \frac{9}{128} \vec{v}_1 \cdot \vec{v}_1 \hat{n} \times \vec{S}_1 \cdot \vec{v}_2 + \frac{9}{32} \vec{v}_1 \cdot \vec{v}_2 \hat{n} \times \vec{S}_1 \cdot \vec{v}_2 + \frac{3}{64} \vec{v}_2 \cdot \vec{v}_2 \hat{n} \times \vec{S}_1 \cdot \vec{v}_1 \right) \Big\}$$

{DiagSet[3, 9, 1], 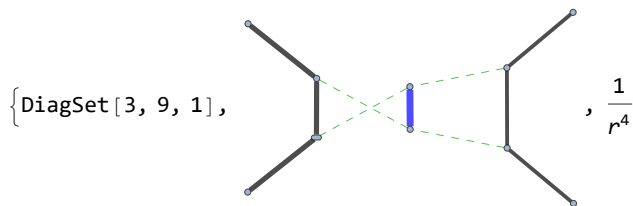,  $\frac{1}{r^4}$

$$G^3 m_1 m_2^2 \left( -64 \hat{n} \cdot \vec{v}_2 \vec{S}_1 \times \vec{v}_1 \cdot \vec{v}_2 - 224 \hat{n} \cdot \vec{v}_1 \hat{n} \cdot \vec{v}_2 \hat{n} \times \vec{S}_1 \cdot \vec{v}_2 + 72 \vec{v}_1 \cdot \vec{v}_2 \hat{n} \times \vec{S}_1 \cdot \vec{v}_2 + \right. \\ \left. \pi^2 \left( \frac{9}{2} \hat{n} \cdot \vec{v}_2 \vec{S}_1 \times \vec{v}_1 \cdot \vec{v}_2 + \frac{45}{2} \hat{n} \cdot \vec{v}_1 \hat{n} \cdot \vec{v}_2 \hat{n} \times \vec{S}_1 \cdot \vec{v}_2 - \frac{9}{2} \vec{v}_1 \cdot \vec{v}_2 \hat{n} \times \vec{S}_1 \cdot \vec{v}_2 \right) + 48 \vec{v}_2 \cdot \vec{v}_2 \hat{n} \times \vec{S}_1 \cdot \vec{v}_1 \right) \Big\}$$

{DiagSet[3, 9, 2], 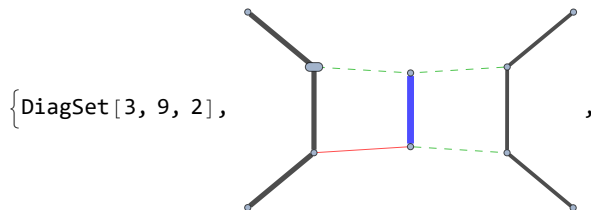,

$$\frac{1}{r^3} G^3 m_1 m_2^2 \left( 164 \hat{n} \cdot \vec{a}_2 \hat{n} \times \vec{S}_1 \cdot \vec{v}_2 - 28 \hat{n} \cdot \vec{v}_2 \hat{n} \times \vec{S}_1 \cdot \vec{a}_2 + \pi^2 \left( -9 \hat{n} \cdot \vec{a}_2 \hat{n} \times \vec{S}_1 \cdot \vec{v}_2 + 3 \hat{n} \cdot \vec{v}_2 \hat{n} \times \vec{S}_1 \cdot \vec{a}_2 + 4 \vec{S}_1 \times \vec{v}_2 \cdot \vec{a}_2 \right) - \right. \\ \left. 64 \vec{S}_1 \times \vec{v}_2 \cdot \vec{a}_2 \right) + \frac{1}{r^4} G^3 m_1 m_2^2 \left( 40 (\hat{n} \cdot \vec{v}_2)^2 \hat{n} \times \vec{S}_1 \cdot \vec{v}_2 + 8 \hat{n} \cdot \vec{v}_2 \vec{S}_1 \times \vec{v}_1 \cdot \vec{v}_2 - 72 \hat{n} \cdot \vec{v}_1 \hat{n} \cdot \vec{v}_2 \hat{n} \times \vec{S}_1 \cdot \vec{v}_2 + \right. \\ \left. \pi^2 \left( \frac{3}{2} \hat{n} \cdot \vec{v}_2 \vec{S}_1 \times \vec{v}_1 \cdot \vec{v}_2 + \frac{15}{2} \hat{n} \cdot \vec{v}_1 \hat{n} \cdot \vec{v}_2 \hat{n} \times \vec{S}_1 \cdot \vec{v}_2 - \frac{3}{2} \vec{v}_1 \cdot \vec{v}_2 \hat{n} \times \vec{S}_1 \cdot \vec{v}_2 \right) - \right. \\ \left. 16 \vec{v}_2 \cdot \vec{v}_2 \hat{n} \times \vec{S}_1 \cdot \vec{v}_1 + 32 \vec{v}_2 \cdot \vec{v}_2 \hat{n} \times \vec{S}_1 \cdot \vec{v}_2 \right) \Big\}$$

{DiagSet[3, 9, 3], 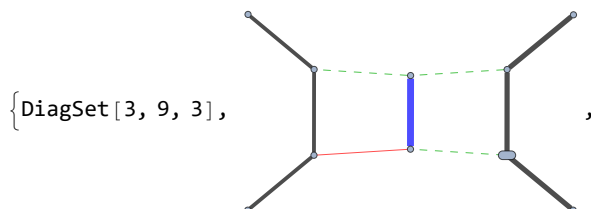,

$$\frac{1}{r^4} G^3 m_1 m_2^2 \left( -76 (\hat{n} \cdot \vec{v}_1)^2 \hat{n} \times \vec{S}_1 \cdot \vec{v}_2 - 12 \hat{n} \cdot \vec{v}_1 \vec{S}_1 \times \vec{v}_1 \cdot \vec{v}_2 - 148 \hat{n} \cdot \vec{v}_2 \hat{n} \cdot \vec{v}_1 \hat{n} \times \vec{S}_1 \cdot \vec{v}_1 + \right. \\ 96 \hat{n} \cdot \vec{v}_2 \hat{n} \cdot \vec{v}_1 \hat{n} \times \vec{S}_1 \cdot \vec{v}_2 + 128 (\hat{n} \cdot \vec{v}_2)^2 \hat{n} \times \vec{S}_1 \cdot \vec{v}_1 - 24 \hat{n} \cdot \vec{v}_2 \vec{S}_1 \times \vec{v}_1 \cdot \vec{v}_2 + \\ 28 \vec{v}_1 \cdot \vec{v}_1 \hat{n} \times \vec{S}_1 \cdot \vec{v}_2 + 76 \vec{v}_1 \cdot \vec{v}_2 \hat{n} \times \vec{S}_1 \cdot \vec{v}_1 - 48 \vec{v}_1 \cdot \vec{v}_2 \hat{n} \times \vec{S}_1 \cdot \vec{v}_2 - 48 \vec{v}_2 \cdot \vec{v}_2 \hat{n} \times \vec{S}_1 \cdot \vec{v}_1 + \\ \left. \pi^2 \left( \frac{15}{2} (\hat{n} \cdot \vec{v}_1)^2 \hat{n} \times \vec{S}_1 \cdot \vec{v}_2 + 15 \hat{n} \cdot \vec{v}_2 \hat{n} \cdot \vec{v}_1 \hat{n} \times \vec{S}_1 \cdot \vec{v}_1 - \frac{15}{2} \hat{n} \cdot \vec{v}_2 \hat{n} \cdot \vec{v}_1 \hat{n} \times \vec{S}_1 \cdot \vec{v}_2 - 15 (\hat{n} \cdot \vec{v}_2)^2 \hat{n} \times \vec{S}_1 \cdot \vec{v}_1 + \right. \right.$$

$$\frac{9}{2} \hat{n} \cdot \vec{v}_2 \vec{S}_1 \times \vec{v}_1 \cdot \vec{v}_2 - \frac{3}{2} \vec{v}_1 \cdot \vec{v}_1 \hat{n} \times \vec{S}_1 \cdot \vec{v}_2 - 3 \vec{v}_1 \cdot \vec{v}_2 \hat{n} \times \vec{S}_1 \cdot \vec{v}_1 + \frac{3}{2} \vec{v}_1 \cdot \vec{v}_2 \hat{n} \times \vec{S}_1 \cdot \vec{v}_2 + 3 \vec{v}_2 \cdot \vec{v}_2 \hat{n} \times \vec{S}_1 \cdot \vec{v}_1 \Big) + \frac{1}{r^3} G^3 m_1 m_2^2 \left( 28 \hat{n} \cdot \vec{v}_1 \hat{n} \times \vec{S}_1 \cdot \vec{v}_2 + 36 \hat{n} \cdot \vec{v}_2 \hat{n} \times \vec{S}_1 \cdot \vec{v}_1 + \pi^2 \left( -3 \hat{n} \cdot \vec{v}_1 \hat{n} \times \vec{S}_1 \cdot \vec{v}_2 - 3 \hat{n} \cdot \vec{v}_2 \hat{n} \times \vec{S}_1 \cdot \vec{v}_1 \right) + 8 \vec{S}_1 \times \vec{v}_1 \cdot \vec{v}_2 \right) \Big\}$$

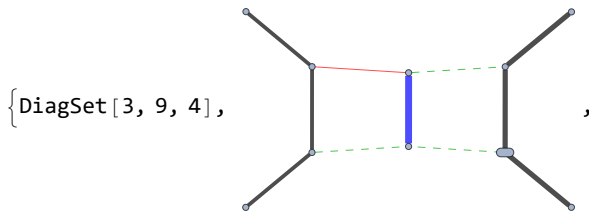

$$\frac{1}{r^3} G^3 m_1 m_2^2 \left( -148 \hat{n} \cdot \vec{a}_1 \hat{n} \times \vec{S}_1 \cdot \vec{v}_2 + 12 \hat{n} \cdot \vec{v}_2 \hat{n} \times \vec{S}_1 \cdot \vec{a}_1 + \pi^2 \left( 9 \hat{n} \cdot \vec{a}_1 \hat{n} \times \vec{S}_1 \cdot \vec{v}_2 + 3 \hat{n} \cdot \vec{v}_2 \hat{n} \times \vec{S}_1 \cdot \vec{a}_1 + 2 \vec{S}_1 \times \vec{a}_1 \cdot \vec{v}_2 \right) - 64 \vec{S}_1 \times \vec{a}_1 \cdot \vec{v}_2 \right) + \frac{1}{r^4} G^3 m_1 m_2^2 \left( 104 (\hat{n} \cdot \vec{v}_1)^2 \hat{n} \times \vec{S}_1 \cdot \vec{v}_2 + 40 \hat{n} \cdot \vec{v}_1 \vec{S}_1 \times \vec{v}_1 \cdot \vec{v}_2 - 32 \hat{n} \cdot \vec{v}_2 \hat{n} \cdot \vec{v}_1 \hat{n} \times \vec{S}_1 \cdot \vec{v}_1 - 52 \hat{n} \cdot \vec{v}_2 \hat{n} \cdot \vec{v}_1 \hat{n} \times \vec{S}_1 \cdot \vec{v}_2 + 12 (\hat{n} \cdot \vec{v}_2)^2 \hat{n} \times \vec{S}_1 \cdot \vec{v}_1 - 20 \hat{n} \cdot \vec{v}_2 \vec{S}_1 \times \vec{v}_1 \cdot \vec{v}_2 - 8 \vec{v}_1 \cdot \vec{v}_1 \hat{n} \times \vec{S}_1 \cdot \vec{v}_2 + \pi^2 \left( -\frac{15}{2} (\hat{n} \cdot \vec{v}_1)^2 \hat{n} \times \vec{S}_1 \cdot \vec{v}_2 - 3 \hat{n} \cdot \vec{v}_1 \vec{S}_1 \times \vec{v}_1 \cdot \vec{v}_2 + \frac{3}{2} \vec{v}_1 \cdot \vec{v}_1 \hat{n} \times \vec{S}_1 \cdot \vec{v}_2 \right) + 24 \vec{v}_1 \cdot \vec{v}_2 \hat{n} \times \vec{S}_1 \cdot \vec{v}_1 - 4 \vec{v}_1 \cdot \vec{v}_2 \hat{n} \times \vec{S}_1 \cdot \vec{v}_2 - 28 \vec{v}_2 \cdot \vec{v}_2 \hat{n} \times \vec{S}_1 \cdot \vec{v}_1 \right) \Big\}$$

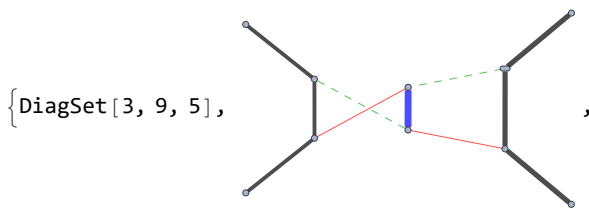

$$\frac{\left( 3 \pi^2 \hat{n} \times \vec{S}_1 \cdot \vec{a}_2 - 44 \hat{n} \times \vec{S}_1 \cdot \vec{a}_2 \right) m_1 m_2^2 G^3}{r^2} + \frac{1}{r^3} \left( 16 \vec{S}_1 \times \vec{v}_1 \cdot \vec{v}_2 + 28 \vec{S}_1 \times \vec{v}_1 \cdot \vec{a}_2 - 24 \vec{S}_1 \times \vec{v}_2 \cdot \vec{a}_2 + 32 \hat{n} \times \vec{S}_1 \cdot \vec{v}_1 \hat{n} \cdot \vec{a}_2 - 36 \hat{n} \times \vec{S}_1 \cdot \vec{v}_2 \hat{n} \cdot \vec{a}_2 + 44 \hat{n} \times \vec{S}_1 \cdot \vec{v}_2 \hat{n} \cdot \vec{v}_1 + 100 \hat{n} \times \vec{S}_1 \cdot \vec{a}_2 \hat{n} \cdot \vec{v}_1 - 36 \hat{n} \times \vec{S}_1 \cdot \vec{v}_1 \hat{n} \cdot \vec{v}_2 - 4 \hat{n} \times \vec{S}_1 \cdot \vec{v}_2 \hat{n} \cdot \vec{v}_2 - 92 \hat{n} \times \vec{S}_1 \cdot \vec{a}_2 \hat{n} \cdot \vec{v}_2 + \pi^2 \left( -2 \vec{S}_1 \times \vec{v}_1 \cdot \vec{v}_2 - \frac{3}{2} \vec{S}_1 \times \vec{v}_1 \cdot \vec{a}_2 - \frac{3}{2} \hat{n} \times \vec{S}_1 \cdot \vec{v}_1 \hat{n} \cdot \vec{a}_2 + 3 \hat{n} \times \vec{S}_1 \cdot \vec{v}_2 \hat{n} \cdot \vec{a}_2 - 3 \hat{n} \times \vec{S}_1 \cdot \vec{v}_2 \hat{n} \cdot \vec{v}_1 - 6 \hat{n} \times \vec{S}_1 \cdot \vec{a}_2 \hat{n} \cdot \vec{v}_1 + 3 \hat{n} \times \vec{S}_1 \cdot \vec{v}_1 \hat{n} \cdot \vec{v}_2 + 3 \hat{n} \times \vec{S}_1 \cdot \vec{a}_2 \hat{n} \cdot \vec{v}_2 \right) \right) m_1 m_2^2 G^3 + \frac{1}{r^4} \left( -86 \hat{n} \times \vec{S}_1 \cdot \vec{v}_2 (\hat{n} \cdot \vec{v}_1)^2 - 44 \vec{S}_1 \times \vec{v}_1 \cdot \vec{v}_2 \hat{n} \cdot \vec{v}_1 + 48 \hat{n} \times \vec{S}_1 \cdot \vec{v}_1 \hat{n} \cdot \vec{v}_2 \hat{n} \cdot \vec{v}_1 + 88 \hat{n} \times \vec{S}_1 \cdot \vec{v}_2 \hat{n} \cdot \vec{v}_2 \hat{n} \cdot \vec{v}_1 - 66 \hat{n} \times \vec{S}_1 \cdot \vec{v}_1 (\hat{n} \cdot \vec{v}_2)^2 - 4 \hat{n} \times \vec{S}_1 \cdot \vec{v}_2 (\hat{n} \cdot \vec{v}_2)^2 + 36 \vec{S}_1 \times \vec{v}_1 \cdot \vec{v}_2 \hat{n} \cdot \vec{v}_2 - 2 \hat{n} \times \vec{S}_1 \cdot \vec{v}_2 \vec{v}_1 \cdot \vec{v}_1 - 16 \hat{n} \times \vec{S}_1 \cdot \vec{v}_1 \vec{v}_1 \cdot \vec{v}_2 + 8 \hat{n} \times \vec{S}_1 \cdot \vec{v}_2 \vec{v}_1 \cdot \vec{v}_2 + 26 \hat{n} \times \vec{S}_1 \cdot \vec{v}_1 \vec{v}_2 \cdot \vec{v}_2 - 28 \hat{n} \times \vec{S}_1 \cdot \vec{v}_2 \vec{v}_2 \cdot \vec{v}_2 + \pi^2 \left( \frac{45}{8} \hat{n} \times \vec{S}_1 \cdot \vec{v}_2 (\hat{n} \cdot \vec{v}_1)^2 + 3 \vec{S}_1 \times \vec{v}_1 \cdot \vec{v}_2 \hat{n} \cdot \vec{v}_1 - \frac{15}{4} \hat{n} \times \vec{S}_1 \cdot \vec{v}_1 \hat{n} \cdot \vec{v}_2 \hat{n} \cdot \vec{v}_1 - \frac{15}{4} \hat{n} \times \vec{S}_1 \cdot \vec{v}_2 \hat{n} \cdot \vec{v}_2 \hat{n} \cdot \vec{v}_1 + \frac{45}{8} \hat{n} \times \vec{S}_1 \cdot \vec{v}_1 (\hat{n} \cdot \vec{v}_2)^2 - \frac{15}{4} \hat{n} \times \vec{S}_1 \cdot \vec{v}_2 (\hat{n} \cdot \vec{v}_2)^2 - 3 \vec{S}_1 \times \vec{v}_1 \cdot \vec{v}_2 \hat{n} \cdot \vec{v}_2 - \frac{9}{8} \hat{n} \times \vec{S}_1 \cdot \vec{v}_2 \vec{v}_1 \cdot \vec{v}_1 + \frac{3}{4} \hat{n} \times \vec{S}_1 \cdot \vec{v}_1 \vec{v}_1 \cdot \vec{v}_2 + \frac{3}{4} \hat{n} \times \vec{S}_1 \cdot \vec{v}_2 \vec{v}_1 \cdot \vec{v}_2 - \frac{9}{8} \hat{n} \times \vec{S}_1 \cdot \vec{v}_1 \vec{v}_2 \cdot \vec{v}_2 + \frac{3}{4} \hat{n} \times \vec{S}_1 \cdot \vec{v}_2 \vec{v}_2 \cdot \vec{v}_2 \right) \right) m_1 m_2^2 G^3 \Big\}$$

{DiagSet[3, 9, 6],

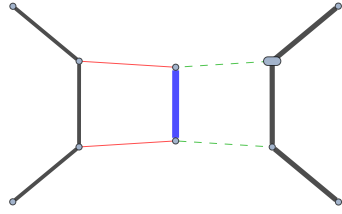

,

$$\frac{\left(40 \hat{n} \times \vec{S}_1 \cdot \vec{a}_1 - 2 \pi^2 \hat{n} \times \vec{S}_1 \cdot \vec{a}_1\right) m_1 m_2^2 G^3}{r^2} + \frac{1}{r^3} \left(-20 \vec{S}_1 \times \vec{v}_1 \cdot \vec{v}_2 - 32 \vec{S}_1 \times \vec{a}_1 \cdot \vec{v}_2 - 24 \vec{S}_1 \times \vec{v}_1 \cdot \vec{a}_1 - \right. \\ \left.36 \hat{n} \times \vec{S}_1 \cdot \vec{v}_1 \hat{n} \cdot \vec{a}_1 + 20 \hat{n} \times \vec{S}_1 \cdot \vec{v}_2 \hat{n} \cdot \vec{a}_1 - 8 \hat{n} \times \vec{S}_1 \cdot \vec{v}_1 \hat{n} \cdot \vec{v}_1 - 40 \hat{n} \times \vec{S}_1 \cdot \vec{v}_2 \hat{n} \cdot \vec{v}_1 - 76 \hat{n} \times \vec{S}_1 \cdot \vec{a}_1 \hat{n} \cdot \vec{v}_1 + \right. \\ \left.44 \hat{n} \times \vec{S}_1 \cdot \vec{v}_1 \hat{n} \cdot \vec{v}_2 + 108 \hat{n} \times \vec{S}_1 \cdot \vec{a}_1 \hat{n} \cdot \vec{v}_2 + \pi^2 \left(2 \vec{S}_1 \times \vec{v}_1 \cdot \vec{v}_2 + 3 \vec{S}_1 \times \vec{a}_1 \cdot \vec{v}_2 + 3 \hat{n} \times \vec{S}_1 \cdot \vec{v}_1 \hat{n} \cdot \vec{a}_1 + \right. \right. \\ \left.3 \hat{n} \times \vec{S}_1 \cdot \vec{v}_2 \hat{n} \cdot \vec{v}_1 + 3 \hat{n} \times \vec{S}_1 \cdot \vec{a}_1 \hat{n} \cdot \vec{v}_1 - 3 \hat{n} \times \vec{S}_1 \cdot \vec{v}_1 \hat{n} \cdot \vec{v}_2 - 9 \hat{n} \times \vec{S}_1 \cdot \vec{a}_1 \hat{n} \cdot \vec{v}_2\right)\right) m_1 m_2^2 G^3 + \\ \frac{1}{r^4} \left(38 \hat{n} \times \vec{S}_1 \cdot \vec{v}_1 (\hat{n} \cdot \vec{v}_1)^2 + 66 \hat{n} \times \vec{S}_1 \cdot \vec{v}_2 (\hat{n} \cdot \vec{v}_1)^2 + 44 \vec{S}_1 \times \vec{v}_1 \cdot \vec{v}_2 \hat{n} \cdot \vec{v}_1 - 88 \hat{n} \times \vec{S}_1 \cdot \vec{v}_1 \hat{n} \cdot \vec{v}_2 \hat{n} \cdot \vec{v}_1 - \right. \\ \left.84 \hat{n} \times \vec{S}_1 \cdot \vec{v}_2 \hat{n} \cdot \vec{v}_2 \hat{n} \cdot \vec{v}_1 + 88 \hat{n} \times \vec{S}_1 \cdot \vec{v}_1 (\hat{n} \cdot \vec{v}_2)^2 - 52 \vec{S}_1 \times \vec{v}_1 \cdot \vec{v}_2 \hat{n} \cdot \vec{v}_2 + 18 \hat{n} \times \vec{S}_1 \cdot \vec{v}_1 \vec{v}_1 \cdot \vec{v}_1 - \right. \\ \left.18 \hat{n} \times \vec{S}_1 \cdot \vec{v}_2 \vec{v}_1 \cdot \vec{v}_1 - 16 \hat{n} \times \vec{S}_1 \cdot \vec{v}_1 \vec{v}_1 \cdot \vec{v}_2 + 20 \hat{n} \times \vec{S}_1 \cdot \vec{v}_2 \vec{v}_1 \cdot \vec{v}_2 + 8 \hat{n} \times \vec{S}_1 \cdot \vec{v}_1 \vec{v}_2 \cdot \vec{v}_2 + \right. \\ \left.\pi^2 \left(-\frac{15}{8} \hat{n} \times \vec{S}_1 \cdot \vec{v}_1 (\hat{n} \cdot \vec{v}_1)^2 - \frac{45}{8} \hat{n} \times \vec{S}_1 \cdot \vec{v}_2 (\hat{n} \cdot \vec{v}_1)^2 - 3 \vec{S}_1 \times \vec{v}_1 \cdot \vec{v}_2 \hat{n} \cdot \vec{v}_1 + \frac{15}{4} \hat{n} \times \vec{S}_1 \cdot \vec{v}_1 \hat{n} \cdot \vec{v}_2 \hat{n} \cdot \vec{v}_1 + \right. \right. \\ \left.\frac{15}{2} \hat{n} \times \vec{S}_1 \cdot \vec{v}_2 \hat{n} \cdot \vec{v}_2 \hat{n} \cdot \vec{v}_1 - \frac{15}{4} \hat{n} \times \vec{S}_1 \cdot \vec{v}_1 (\hat{n} \cdot \vec{v}_2)^2 + 3 \vec{S}_1 \times \vec{v}_1 \cdot \vec{v}_2 \hat{n} \cdot \vec{v}_2 + \frac{3}{8} \hat{n} \times \vec{S}_1 \cdot \vec{v}_1 \vec{v}_1 \cdot \vec{v}_1 + \right. \\ \left.\frac{9}{8} \hat{n} \times \vec{S}_1 \cdot \vec{v}_2 \vec{v}_1 \cdot \vec{v}_1 - \frac{3}{4} \hat{n} \times \vec{S}_1 \cdot \vec{v}_1 \vec{v}_1 \cdot \vec{v}_2 - \frac{3}{2} \hat{n} \times \vec{S}_1 \cdot \vec{v}_2 \vec{v}_1 \cdot \vec{v}_2 + \frac{3}{4} \hat{n} \times \vec{S}_1 \cdot \vec{v}_1 \vec{v}_2 \cdot \vec{v}_2\right)\right) m_1 m_2^2 G^3 \Big\}$$

{DiagSet[3, 9, 7],

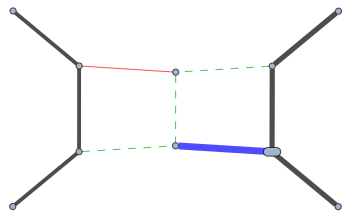

,  $\frac{1}{r^4} G^3 m_1 m_2^2$ ,

$$\left(20 (\hat{n} \cdot \vec{v}_1)^2 \hat{n} \times \vec{S}_1 \cdot \vec{v}_2 + 4 \hat{n} \cdot \vec{v}_1 \vec{S}_1 \times \vec{v}_1 \cdot \vec{v}_2 - 40 \hat{n} \cdot \vec{v}_2 \hat{n} \cdot \vec{v}_1 \hat{n} \times \vec{S}_1 \cdot \vec{v}_1 - 24 \vec{v}_1 \cdot \vec{v}_1 \hat{n} \times \vec{S}_1 \cdot \vec{v}_2 + 24 \vec{v}_1 \cdot \vec{v}_2 \hat{n} \times \vec{S}_1 \cdot \vec{v}_1\right) \Big\}$$

{DiagSet[3, 9, 8],

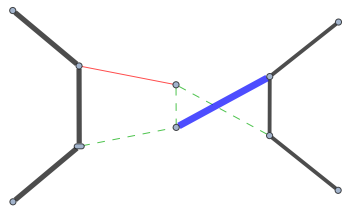

,  $\frac{1}{r^4}$

$$G^3 m_1 m_2^2 \left(28 (\hat{n} \cdot \vec{v}_2)^2 \hat{n} \times \vec{S}_1 \cdot \vec{v}_2 - 8 \vec{v}_2 \cdot \vec{v}_2 \hat{n} \times \vec{S}_1 \cdot \vec{v}_2 + \pi^2 \left(\frac{75}{4} (\hat{n} \cdot \vec{v}_2)^2 \hat{n} \times \vec{S}_1 \cdot \vec{v}_2 - \frac{15}{4} \vec{v}_2 \cdot \vec{v}_2 \hat{n} \times \vec{S}_1 \cdot \vec{v}_2\right)\right) \Big\}$$

{DiagSet[3, 9, 9],

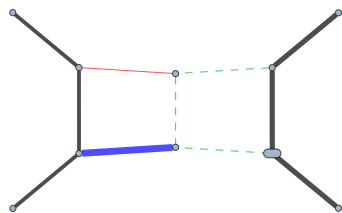

,  $\frac{1}{r^4}$

$$G^3 m_1 m_2^2 \left( -64 (\hat{n} \cdot \vec{v}_2)^2 \hat{n} \times \vec{S}_1 \cdot \vec{v}_1 + 36 \hat{n} \cdot \vec{v}_2 \vec{S}_1 \times \vec{v}_1 \cdot \vec{v}_2 + 36 \hat{n} \cdot \vec{v}_1 \hat{n} \cdot \vec{v}_2 \hat{n} \times \vec{S}_1 \cdot \vec{v}_2 + \right. \\ \left. 8 \vec{v}_2 \cdot \vec{v}_2 \hat{n} \times \vec{S}_1 \cdot \vec{v}_1 + \pi^2 \left( \frac{15}{4} (\hat{n} \cdot \vec{v}_2)^2 \hat{n} \times \vec{S}_1 \cdot \vec{v}_1 - 3 \hat{n} \cdot \vec{v}_2 \vec{S}_1 \times \vec{v}_1 \cdot \vec{v}_2 - \right. \right. \\ \left. \left. \frac{15}{2} \hat{n} \cdot \vec{v}_1 \hat{n} \cdot \vec{v}_2 \hat{n} \times \vec{S}_1 \cdot \vec{v}_2 + \frac{3}{2} \vec{v}_1 \cdot \vec{v}_2 \hat{n} \times \vec{S}_1 \cdot \vec{v}_2 - \frac{3}{4} \vec{v}_2 \cdot \vec{v}_2 \hat{n} \times \vec{S}_1 \cdot \vec{v}_1 \right) \right) \Bigg\}$$

$$\left\{ \text{DiagSet}[3, 9, 10], \frac{1}{r^3} G^3 m_1 m_2^2 \left( -8 \hat{n} \cdot \vec{a}_2 \hat{n} \times \vec{S}_1 \cdot \vec{v}_2 + 8 \hat{n} \cdot \vec{v}_2 \hat{n} \times \vec{S}_1 \cdot \vec{a}_2 + \right. \right.$$
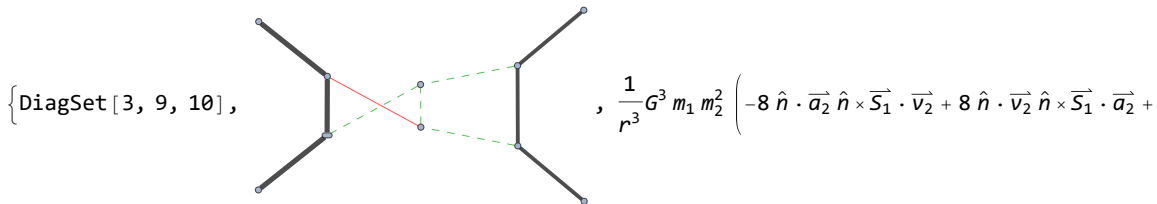

$$\pi^2 \left( -\frac{3}{2} \hat{n} \cdot \vec{a}_2 \hat{n} \times \vec{S}_1 \cdot \vec{v}_2 - 15 \hat{n} \cdot \vec{v}_2 \hat{n} \times \vec{S}_1 \cdot \vec{a}_2 - \frac{9}{2} \vec{S}_1 \times \vec{v}_2 \cdot \vec{a}_2 + \frac{15}{2} \hat{n} \cdot \vec{v}_2 \hat{n} \times \vec{S}_1 \cdot \vec{v}_2 \right) - 16 \vec{S}_1 \times \vec{v}_2 \cdot \vec{a}_2 \Bigg) + \\ \frac{1}{r^4} G^3 m_1 m_2^2 \left( 55 (\hat{n} \cdot \vec{v}_2)^2 \hat{n} \times \vec{S}_1 \cdot \vec{v}_1 - 21 (\hat{n} \cdot \vec{v}_2)^2 \hat{n} \times \vec{S}_1 \cdot \vec{v}_2 - 40 \hat{n} \cdot \vec{v}_2 \vec{S}_1 \times \vec{v}_1 \cdot \vec{v}_2 - \right. \\ \left. 30 \hat{n} \cdot \vec{v}_1 \hat{n} \cdot \vec{v}_2 \hat{n} \times \vec{S}_1 \cdot \vec{v}_2 + 14 \vec{v}_1 \cdot \vec{v}_2 \hat{n} \times \vec{S}_1 \cdot \vec{v}_2 - 3 \vec{v}_2 \cdot \vec{v}_2 \hat{n} \times \vec{S}_1 \cdot \vec{v}_1 - 11 \vec{v}_2 \cdot \vec{v}_2 \hat{n} \times \vec{S}_1 \cdot \vec{v}_2 + \right. \\ \left. \pi^2 \left( -\frac{135}{16} (\hat{n} \cdot \vec{v}_2)^2 \hat{n} \times \vec{S}_1 \cdot \vec{v}_1 - \frac{615}{16} (\hat{n} \cdot \vec{v}_2)^2 \hat{n} \times \vec{S}_1 \cdot \vec{v}_2 - \frac{3}{4} \hat{n} \cdot \vec{v}_2 \vec{S}_1 \times \vec{v}_1 \cdot \vec{v}_2 - \right. \right. \\ \left. \left. \frac{165}{8} \hat{n} \cdot \vec{v}_1 \hat{n} \cdot \vec{v}_2 \hat{n} \times \vec{S}_1 \cdot \vec{v}_2 + \frac{33}{8} \vec{v}_1 \cdot \vec{v}_2 \hat{n} \times \vec{S}_1 \cdot \vec{v}_2 + \frac{27}{16} \vec{v}_2 \cdot \vec{v}_2 \hat{n} \times \vec{S}_1 \cdot \vec{v}_1 + \frac{123}{16} \vec{v}_2 \cdot \vec{v}_2 \hat{n} \times \vec{S}_1 \cdot \vec{v}_2 \right) \right) \Bigg\}$$

$$\left\{ \text{DiagSet}[3, 9, 11], \right.$$
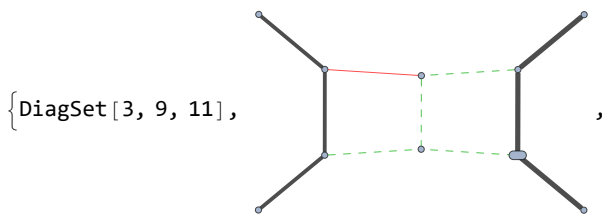

$$\frac{1}{r^3} \left( 8 \vec{S}_1 \times \vec{v}_1 \cdot \vec{v}_2 - 12 \vec{S}_1 \times \vec{a}_1 \cdot \vec{v}_2 + 4 \vec{S}_1 \times \vec{v}_1 \cdot \vec{a}_2 + 8 \hat{n} \times \vec{S}_1 \cdot \vec{v}_1 \hat{n} \cdot \vec{a}_2 + \right. \\ \left. 8 \hat{n} \times \vec{S}_1 \cdot \vec{v}_2 \hat{n} \cdot \vec{v}_1 - 12 \hat{n} \times \vec{S}_1 \cdot \vec{a}_2 \hat{n} \cdot \vec{v}_1 - 8 \hat{n} \times \vec{S}_1 \cdot \vec{v}_1 \hat{n} \cdot \vec{v}_2 + 4 \hat{n} \times \vec{S}_1 \cdot \vec{a}_1 \hat{n} \cdot \vec{v}_2 + \right. \\ \left. \pi^2 \left( \frac{1}{2} \vec{S}_1 \times \vec{v}_1 \cdot \vec{v}_2 + \frac{3}{2} \vec{S}_1 \times \vec{a}_1 \cdot \vec{v}_2 + \frac{3}{2} \hat{n} \times \vec{S}_1 \cdot \vec{v}_2 \hat{n} \cdot \vec{a}_1 + \frac{3}{2} \hat{n} \times \vec{S}_1 \cdot \vec{v}_2 \hat{n} \cdot \vec{v}_1 - 3 \hat{n} \times \vec{S}_1 \cdot \vec{a}_1 \hat{n} \cdot \vec{v}_2 \right) \right) m_1 m_2^2 G^3 + \\ \frac{1}{r^4} \left( -35 \hat{n} \times \vec{S}_1 \cdot \vec{v}_2 (\hat{n} \cdot \vec{v}_1)^2 + 8 \vec{S}_1 \times \vec{v}_1 \cdot \vec{v}_2 \hat{n} \cdot \vec{v}_1 + 10 \hat{n} \times \vec{S}_1 \cdot \vec{v}_1 \hat{n} \cdot \vec{v}_2 \hat{n} \cdot \vec{v}_1 - 22 \hat{n} \times \vec{S}_1 \cdot \vec{v}_2 \hat{n} \cdot \vec{v}_2 \hat{n} \cdot \vec{v}_1 + \right. \\ \left. 43 \hat{n} \times \vec{S}_1 \cdot \vec{v}_1 (\hat{n} \cdot \vec{v}_2)^2 - 36 \vec{S}_1 \times \vec{v}_1 \cdot \vec{v}_2 \hat{n} \cdot \vec{v}_2 + 11 \hat{n} \times \vec{S}_1 \cdot \vec{v}_2 \vec{v}_1 \cdot \vec{v}_1 - 22 \hat{n} \times \vec{S}_1 \cdot \vec{v}_1 \vec{v}_1 \cdot \vec{v}_2 + \right. \\ \left. 10 \hat{n} \times \vec{S}_1 \cdot \vec{v}_2 \vec{v}_1 \cdot \vec{v}_2 + \hat{n} \times \vec{S}_1 \cdot \vec{v}_1 \vec{v}_2 \cdot \vec{v}_2 + \pi^2 \left( -\frac{105}{16} \hat{n} \times \vec{S}_1 \cdot \vec{v}_2 (\hat{n} \cdot \vec{v}_1)^2 - \frac{15}{4} \vec{S}_1 \times \vec{v}_1 \cdot \vec{v}_2 \hat{n} \cdot \vec{v}_1 + \right. \right. \\ \left. \left. \frac{45}{8} \hat{n} \times \vec{S}_1 \cdot \vec{v}_1 \hat{n} \cdot \vec{v}_2 \hat{n} \cdot \vec{v}_1 - \frac{15}{8} \hat{n} \times \vec{S}_1 \cdot \vec{v}_2 \hat{n} \cdot \vec{v}_2 \hat{n} \cdot \vec{v}_1 - \frac{75}{16} \hat{n} \times \vec{S}_1 \cdot \vec{v}_1 (\hat{n} \cdot \vec{v}_2)^2 + \frac{3}{2} \vec{S}_1 \times \vec{v}_1 \cdot \vec{v}_2 \hat{n} \cdot \vec{v}_2 + \right. \right. \\ \left. \left. \frac{21}{16} \hat{n} \times \vec{S}_1 \cdot \vec{v}_2 \vec{v}_1 \cdot \vec{v}_1 - \frac{9}{8} \hat{n} \times \vec{S}_1 \cdot \vec{v}_1 \vec{v}_1 \cdot \vec{v}_2 + \frac{3}{8} \hat{n} \times \vec{S}_1 \cdot \vec{v}_2 \vec{v}_1 \cdot \vec{v}_2 + \frac{15}{16} \hat{n} \times \vec{S}_1 \cdot \vec{v}_1 \vec{v}_2 \cdot \vec{v}_2 \right) \right) m_1 m_2^2 G^3 \Bigg\}$$

$$\left\{ \text{DiagSet}[3, 9, 12], \right.$$
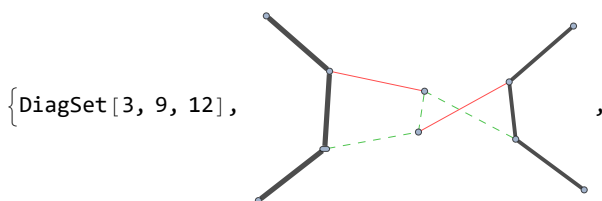



$$\frac{G^3 m_1 m_2^2 \left( 16 \hat{n} \cdot \vec{v}_2 \hat{n} \times \vec{a}_1 \cdot \vec{S}_1 - 16 \vec{a}_1 \times \vec{S}_1 \cdot \vec{v}_2 - 16 \hat{n} \cdot \vec{v}_2 \hat{n} \times \vec{S}_1 \cdot \vec{v}_1 + 16 \vec{S}_1 \times \vec{v}_1 \cdot \vec{v}_2 \right)}{r^3} + \frac{1}{r^4} G^3 m_1 m_2^2 \left( -18 \hat{n} \cdot \vec{v}_1 \vec{S}_1 \times \vec{v}_1 \cdot \vec{v}_2 + 40 \hat{n} \cdot \vec{v}_2 \hat{n} \cdot \vec{v}_1 \hat{n} \times \vec{S}_1 \cdot \vec{v}_1 - 6 \vec{v}_1 \cdot \vec{v}_1 \hat{n} \times \vec{S}_1 \cdot \vec{v}_2 - 22 \vec{v}_1 \cdot \vec{v}_2 \hat{n} \times \vec{S}_1 \cdot \vec{v}_1 - 8 \vec{v}_2 \cdot \vec{v}_2 \hat{n} \times \vec{S}_1 \cdot \vec{v}_2 \right) \Big\}$$

{DiagSet[3, 9, 13],

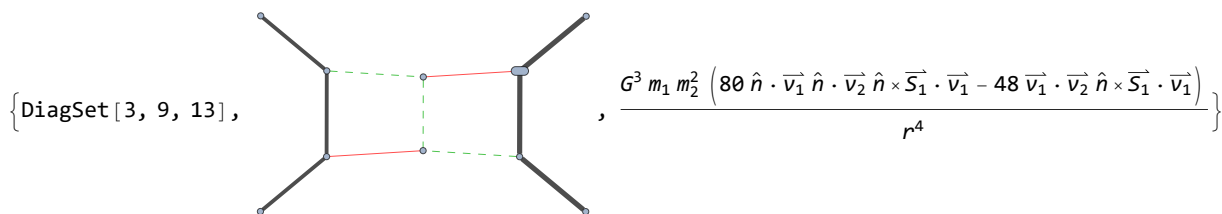

,  $\frac{G^3 m_1 m_2^2 \left( 80 \hat{n} \cdot \vec{v}_1 \hat{n} \cdot \vec{v}_2 \hat{n} \times \vec{S}_1 \cdot \vec{v}_1 - 48 \vec{v}_1 \cdot \vec{v}_2 \hat{n} \times \vec{S}_1 \cdot \vec{v}_1 \right)}{r^4}$  }

{DiagSet[3, 9, 14],

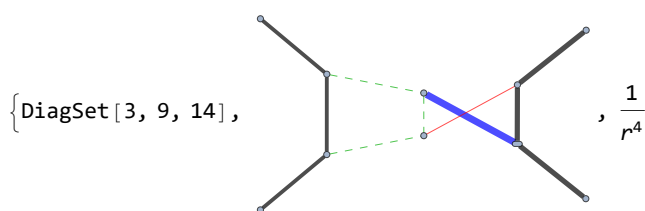

,  $\frac{1}{r^4}$

$$G^3 m_1 m_2^2 \left( 4 \hat{n} \cdot \vec{v}_2 \vec{S}_1 \times \vec{v}_1 \cdot \vec{v}_2 + 20 \hat{n} \cdot \vec{v}_1 \hat{n} \cdot \vec{v}_2 \hat{n} \times \vec{S}_1 \cdot \vec{v}_2 + 28 \vec{v}_1 \cdot \vec{v}_2 \hat{n} \times \vec{S}_1 \cdot \vec{v}_2 - 28 \vec{v}_2 \cdot \vec{v}_2 \hat{n} \times \vec{S}_1 \cdot \vec{v}_1 \right) \Big\}$$

{DiagSet[3, 9, 15],

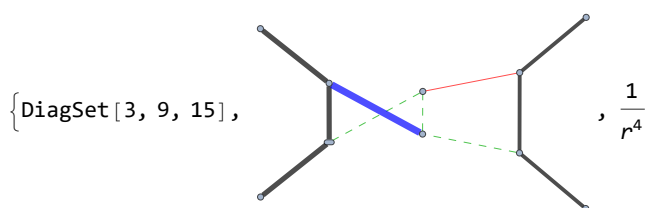

,  $\frac{1}{r^4}$

$$G^3 m_1 m_2^2 \left( 70 \left( \hat{n} \cdot \vec{v}_1 \right)^2 \hat{n} \times \vec{S}_1 \cdot \vec{v}_2 + 8 \hat{n} \cdot \vec{v}_1 \vec{S}_1 \times \vec{v}_1 \cdot \vec{v}_2 + 44 \hat{n} \cdot \vec{v}_2 \hat{n} \cdot \vec{v}_1 \hat{n} \times \vec{S}_1 \cdot \vec{v}_1 - 14 \vec{v}_1 \cdot \vec{v}_1 \hat{n} \times \vec{S}_1 \cdot \vec{v}_2 - 16 \vec{v}_1 \cdot \vec{v}_2 \hat{n} \times \vec{S}_1 \cdot \vec{v}_1 + \pi^2 \left( \frac{75}{8} \left( \hat{n} \cdot \vec{v}_1 \right)^2 \hat{n} \times \vec{S}_1 \cdot \vec{v}_2 + 6 \hat{n} \cdot \vec{v}_1 \vec{S}_1 \times \vec{v}_1 \cdot \vec{v}_2 - \frac{45}{4} \hat{n} \cdot \vec{v}_2 \hat{n} \cdot \vec{v}_1 \hat{n} \times \vec{S}_1 \cdot \vec{v}_1 - \frac{15}{8} \vec{v}_1 \cdot \vec{v}_1 \hat{n} \times \vec{S}_1 \cdot \vec{v}_2 + \frac{9}{4} \vec{v}_1 \cdot \vec{v}_2 \hat{n} \times \vec{S}_1 \cdot \vec{v}_1 \right) \right) \Big\}$$

{DiagSet[3, 9, 16],

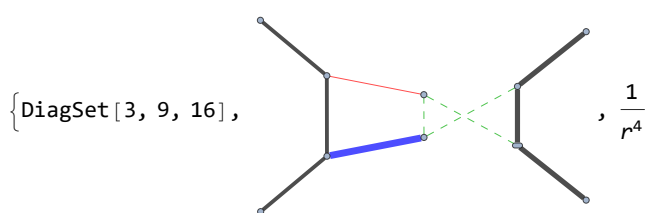

,  $\frac{1}{r^4}$

$$G^3 m_1 m_2^2 \left( -20 \left( \hat{n} \cdot \vec{v}_2 \right)^2 \hat{n} \times \vec{S}_1 \cdot \vec{v}_1 - 8 \hat{n} \cdot \vec{v}_2 \vec{S}_1 \times \vec{v}_1 \cdot \vec{v}_2 - 24 \hat{n} \cdot \vec{v}_1 \hat{n} \cdot \vec{v}_2 \hat{n} \times \vec{S}_1 \cdot \vec{v}_2 + 12 \vec{v}_1 \cdot \vec{v}_2 \hat{n} \times \vec{S}_1 \cdot \vec{v}_2 + 4 \vec{v}_2 \cdot \vec{v}_2 \hat{n} \times \vec{S}_1 \cdot \vec{v}_1 + \pi^2 \left( -\frac{15}{4} \left( \hat{n} \cdot \vec{v}_2 \right)^2 \hat{n} \times \vec{S}_1 \cdot \vec{v}_1 + 3 \hat{n} \cdot \vec{v}_2 \vec{S}_1 \times \vec{v}_1 \cdot \vec{v}_2 + \frac{15}{2} \hat{n} \cdot \vec{v}_1 \hat{n} \cdot \vec{v}_2 \hat{n} \times \vec{S}_1 \cdot \vec{v}_2 - \frac{3}{2} \vec{v}_1 \cdot \vec{v}_2 \hat{n} \times \vec{S}_1 \cdot \vec{v}_2 + \frac{3}{4} \vec{v}_2 \cdot \vec{v}_2 \hat{n} \times \vec{S}_1 \cdot \vec{v}_1 \right) \right) \Big\}$$

{DiagSet[3, 9, 17],

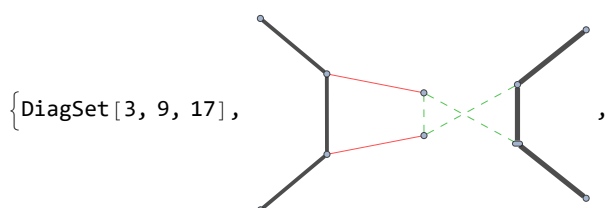

,

$$\frac{G^3 m_1 m_2^2 \left( 16 \hat{n} \cdot \vec{v}_1 \hat{n} \times \vec{S}_1 \cdot \vec{a}_1 + 16 \vec{S}_1 \times \vec{v}_1 \cdot \vec{a}_1 + 16 \hat{n} \cdot \vec{v}_1 \hat{n} \times \vec{S}_1 \cdot \vec{v}_1 \right)}{r^3} +$$

$$\frac{G^3 m_1 m_2^2 \left( -40 (\hat{n} \cdot \vec{v}_1)^2 \hat{n} \times \vec{S}_1 \cdot \vec{v}_1 + 24 \vec{v}_1 \cdot \vec{v}_1 \hat{n} \times \vec{S}_1 \cdot \vec{v}_1 + 12 \vec{v}_2 \cdot \vec{v}_2 \hat{n} \times \vec{S}_1 \cdot \vec{v}_1 \right)}{r^4} \Bigg\}$$

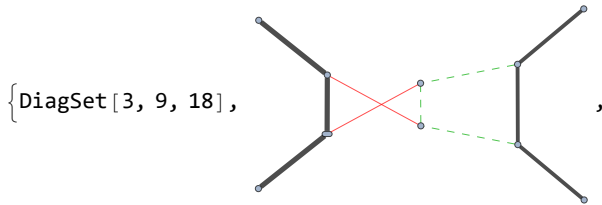

$$\frac{G^3 m_1 m_2^2 \left( -80 (\hat{n} \cdot \vec{v}_2)^2 \hat{n} \times \vec{S}_1 \cdot \vec{v}_1 + 32 \hat{n} \cdot \vec{v}_2 \vec{S}_1 \times \vec{v}_1 \cdot \vec{v}_2 + 48 \vec{v}_2 \cdot \vec{v}_2 \hat{n} \times \vec{S}_1 \cdot \vec{v}_1 \right)}{r^4} \Bigg\}$$

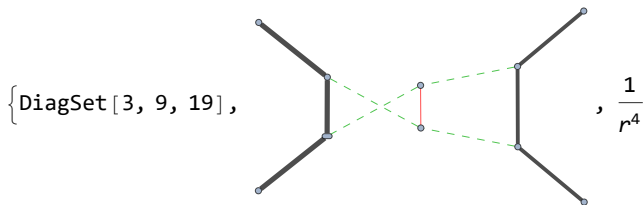

$$G^3 m_1 m_2^2 \left( 80 (\hat{n} \cdot \vec{v}_2)^2 \hat{n} \times \vec{S}_1 \cdot \vec{v}_1 - 48 \hat{n} \cdot \vec{v}_2 \vec{S}_1 \times \vec{v}_1 \cdot \vec{v}_2 - 80 \hat{n} \cdot \vec{v}_1 \hat{n} \cdot \vec{v}_2 \hat{n} \times \vec{S}_1 \cdot \vec{v}_2 + 80 \vec{v}_1 \cdot \vec{v}_2 \hat{n} \times \vec{S}_1 \cdot \vec{v}_2 \right) \Bigg\}$$

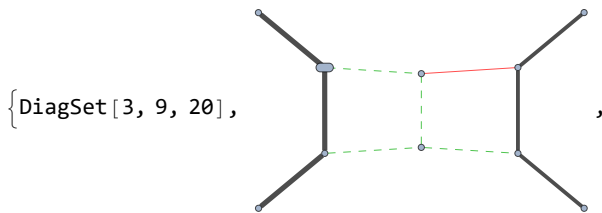

$$\frac{1}{r^3} \left( 12 \vec{S}_1 \times \vec{v}_1 \cdot \vec{v}_2 - 4 \vec{S}_1 \times \vec{a}_1 \cdot \vec{v}_2 + 4 \vec{S}_1 \times \vec{v}_1 \cdot \vec{a}_2 - 20 \hat{n} \times \vec{S}_1 \cdot \vec{v}_2 \hat{n} \cdot \vec{a}_1 - 20 \hat{n} \times \vec{S}_1 \cdot \vec{v}_1 \hat{n} \cdot \vec{a}_2 + \right.$$

$$24 \hat{n} \times \vec{S}_1 \cdot \vec{v}_2 \hat{n} \cdot \vec{v}_1 - 16 \hat{n} \times \vec{S}_1 \cdot \vec{a}_2 \hat{n} \cdot \vec{v}_1 + 12 \hat{n} \times \vec{S}_1 \cdot \vec{v}_1 \hat{n} \cdot \vec{v}_2 - 16 \hat{n} \times \vec{S}_1 \cdot \vec{a}_1 \hat{n} \cdot \vec{v}_2 +$$

$$\pi^2 \left( \frac{3}{2} \vec{S}_1 \times \vec{v}_1 \cdot \vec{v}_2 + \frac{5}{2} \vec{S}_1 \times \vec{a}_1 \cdot \vec{v}_2 - \frac{5}{2} \vec{S}_1 \times \vec{v}_1 \cdot \vec{a}_2 + \frac{9}{2} \hat{n} \times \vec{S}_1 \cdot \vec{v}_2 \hat{n} \cdot \vec{a}_1 + \frac{9}{2} \hat{n} \times \vec{S}_1 \cdot \vec{v}_1 \hat{n} \cdot \vec{a}_2 + \right.$$

$$\left. \frac{3}{2} \hat{n} \times \vec{S}_1 \cdot \vec{v}_2 \hat{n} \cdot \vec{v}_1 - 3 \hat{n} \times \vec{S}_1 \cdot \vec{a}_2 \hat{n} \cdot \vec{v}_1 - 3 \hat{n} \times \vec{S}_1 \cdot \vec{v}_1 \hat{n} \cdot \vec{v}_2 - 3 \hat{n} \times \vec{S}_1 \cdot \vec{a}_1 \hat{n} \cdot \vec{v}_2 \right) \Bigg) m_1 m_2^2 G^3 + \frac{1}{r^4}$$

$$\left( -80 \hat{n} \times \vec{S}_1 \cdot \vec{v}_2 (\hat{n} \cdot \vec{v}_1)^2 - 32 \vec{S}_1 \times \vec{v}_1 \cdot \vec{v}_2 \hat{n} \cdot \vec{v}_1 - 12 \hat{n} \times \vec{S}_1 \cdot \vec{v}_1 \hat{n} \cdot \vec{v}_2 \hat{n} \cdot \vec{v}_1 - 60 \hat{n} \times \vec{S}_1 \cdot \vec{v}_2 \hat{n} \cdot \vec{v}_2 \hat{n} \cdot \vec{v}_1 + \right.$$

$$12 \hat{n} \times \vec{S}_1 \cdot \vec{v}_1 (\hat{n} \cdot \vec{v}_2)^2 + 16 \hat{n} \times \vec{S}_1 \cdot \vec{v}_2 \vec{v}_1 \cdot \vec{v}_1 - 20 \hat{n} \times \vec{S}_1 \cdot \vec{v}_1 \vec{v}_1 \cdot \vec{v}_2 + 32 \hat{n} \times \vec{S}_1 \cdot \vec{v}_2 \vec{v}_1 \cdot \vec{v}_2 +$$

$$\pi^2 \left( -\frac{45}{4} \hat{n} \times \vec{S}_1 \cdot \vec{v}_2 (\hat{n} \cdot \vec{v}_1)^2 - \frac{27}{4} \vec{S}_1 \times \vec{v}_1 \cdot \vec{v}_2 \hat{n} \cdot \vec{v}_1 + \frac{45}{4} \hat{n} \times \vec{S}_1 \cdot \vec{v}_1 \hat{n} \cdot \vec{v}_2 \hat{n} \cdot \vec{v}_1 - \frac{15}{4} \hat{n} \times \vec{S}_1 \cdot \vec{v}_2 \hat{n} \cdot \vec{v}_2 \hat{n} \cdot \vec{v}_1 - \right.$$

$$\left. \frac{3}{4} \vec{S}_1 \times \vec{v}_1 \cdot \vec{v}_2 \hat{n} \cdot \vec{v}_2 + \frac{9}{4} \hat{n} \times \vec{S}_1 \cdot \vec{v}_2 \vec{v}_1 \cdot \vec{v}_1 - \frac{9}{4} \hat{n} \times \vec{S}_1 \cdot \vec{v}_1 \vec{v}_1 \cdot \vec{v}_2 + \frac{3}{4} \hat{n} \times \vec{S}_1 \cdot \vec{v}_2 \vec{v}_1 \cdot \vec{v}_2 \right) \Bigg) m_1 m_2^2 G^3 \Bigg\}$$

{DiagSet[3, 9, 21],

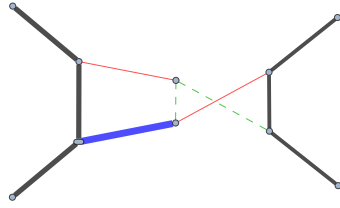

,

$$\frac{1}{r^3} G^3 m_1 m_2^2 \left( 12 \hat{n} \cdot \vec{a}_2 \hat{n} \times \vec{S}_1 \cdot \vec{v}_1 - 12 \hat{n} \cdot \vec{v}_1 \hat{n} \times \vec{S}_1 \cdot \vec{a}_2 + \pi^2 \left( -3 \hat{n} \cdot \vec{v}_1 \hat{n} \times \vec{S}_1 \cdot \vec{a}_2 - \left( \vec{S}_1 \times \vec{v}_1 \cdot \vec{a}_2 \right) \right) \right) + \frac{1}{r^4} G^3 m_1 m_2^2 \left( 23 \left( \hat{n} \cdot \vec{v}_1 \right)^2 \hat{n} \times \vec{S}_1 \cdot \vec{v}_2 - 8 \hat{n} \cdot \vec{v}_1 \vec{S}_1 \times \vec{v}_1 \cdot \vec{v}_2 - 22 \hat{n} \cdot \vec{v}_2 \hat{n} \cdot \vec{v}_1 \hat{n} \times \vec{S}_1 \cdot \vec{v}_1 - 62 \hat{n} \cdot \vec{v}_2 \hat{n} \cdot \vec{v}_1 \hat{n} \times \vec{S}_1 \cdot \vec{v}_2 + 61 \left( \hat{n} \cdot \vec{v}_2 \right)^2 \hat{n} \times \vec{S}_1 \cdot \vec{v}_1 - 12 \hat{n} \cdot \vec{v}_2 \vec{S}_1 \times \vec{v}_1 \cdot \vec{v}_2 - 7 \vec{v}_1 \cdot \vec{v}_1 \hat{n} \times \vec{S}_1 \cdot \vec{v}_2 + 2 \vec{v}_1 \cdot \vec{v}_2 \hat{n} \times \vec{S}_1 \cdot \vec{v}_1 + 6 \vec{v}_1 \cdot \vec{v}_2 \hat{n} \times \vec{S}_1 \cdot \vec{v}_2 - 5 \vec{v}_2 \cdot \vec{v}_2 \hat{n} \times \vec{S}_1 \cdot \vec{v}_1 + \pi^2 \left( \frac{45}{16} \left( \hat{n} \cdot \vec{v}_1 \right)^2 \hat{n} \times \vec{S}_1 \cdot \vec{v}_2 + \frac{3}{2} \hat{n} \cdot \vec{v}_1 \vec{S}_1 \times \vec{v}_1 \cdot \vec{v}_2 - \frac{15}{8} \hat{n} \cdot \vec{v}_2 \hat{n} \cdot \vec{v}_1 \hat{n} \times \vec{S}_1 \cdot \vec{v}_1 - \frac{15}{8} \hat{n} \cdot \vec{v}_2 \hat{n} \cdot \vec{v}_1 \hat{n} \times \vec{S}_1 \cdot \vec{v}_2 + \frac{15}{16} \left( \hat{n} \cdot \vec{v}_2 \right)^2 \hat{n} \times \vec{S}_1 \cdot \vec{v}_1 - \frac{3}{4} \hat{n} \cdot \vec{v}_2 \vec{S}_1 \times \vec{v}_1 \cdot \vec{v}_2 - \frac{9}{16} \vec{v}_1 \cdot \vec{v}_1 \hat{n} \times \vec{S}_1 \cdot \vec{v}_2 + \frac{3}{8} \vec{v}_1 \cdot \vec{v}_2 \hat{n} \times \vec{S}_1 \cdot \vec{v}_1 + \frac{3}{8} \vec{v}_1 \cdot \vec{v}_2 \hat{n} \times \vec{S}_1 \cdot \vec{v}_2 - \frac{3}{16} \vec{v}_2 \cdot \vec{v}_2 \hat{n} \times \vec{S}_1 \cdot \vec{v}_1 \right) \right) \Bigg\}$$

{DiagSet[3, 9, 22],

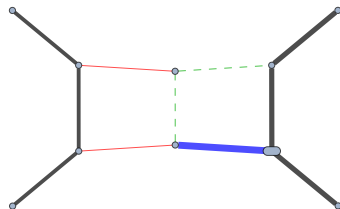

,

$$\frac{1}{r^3} G^3 m_1 m_2^2 \left( -12 \hat{n} \cdot \vec{a}_1 \hat{n} \times \vec{S}_1 \cdot \vec{v}_1 + 12 \hat{n} \cdot \vec{v}_1 \hat{n} \times \vec{S}_1 \cdot \vec{a}_1 + \pi^2 \left( -3 \hat{n} \cdot \vec{v}_1 \hat{n} \times \vec{S}_1 \cdot \vec{a}_1 - \left( \vec{S}_1 \times \vec{v}_1 \cdot \vec{a}_1 \right) \right) \right) + \frac{1}{r^4} G^3 m_1 m_2^2 \left( \left( \hat{n} \cdot \vec{v}_1 \right)^2 \left( - \left( \hat{n} \times \vec{S}_1 \cdot \vec{v}_1 \right) \right) + 19 \left( \hat{n} \cdot \vec{v}_1 \right)^2 \hat{n} \times \vec{S}_1 \cdot \vec{v}_2 + 12 \hat{n} \cdot \vec{v}_1 \vec{S}_1 \times \vec{v}_1 \cdot \vec{v}_2 - 18 \hat{n} \cdot \vec{v}_2 \hat{n} \cdot \vec{v}_1 \hat{n} \times \vec{S}_1 \cdot \vec{v}_1 + 5 \vec{v}_1 \cdot \vec{v}_1 \hat{n} \times \vec{S}_1 \cdot \vec{v}_1 + \vec{v}_1 \cdot \vec{v}_1 \hat{n} \times \vec{S}_1 \cdot \vec{v}_2 - 2 \vec{v}_1 \cdot \vec{v}_2 \hat{n} \times \vec{S}_1 \cdot \vec{v}_1 + \pi^2 \left( \frac{105}{16} \left( \hat{n} \cdot \vec{v}_1 \right)^2 \hat{n} \times \vec{S}_1 \cdot \vec{v}_1 - \frac{15}{16} \left( \hat{n} \cdot \vec{v}_1 \right)^2 \hat{n} \times \vec{S}_1 \cdot \vec{v}_2 + \frac{3}{4} \hat{n} \cdot \vec{v}_1 \vec{S}_1 \times \vec{v}_1 \cdot \vec{v}_2 - \frac{45}{8} \hat{n} \cdot \vec{v}_2 \hat{n} \cdot \vec{v}_1 \hat{n} \times \vec{S}_1 \cdot \vec{v}_1 - \frac{21}{16} \vec{v}_1 \cdot \vec{v}_1 \hat{n} \times \vec{S}_1 \cdot \vec{v}_1 + \frac{3}{16} \vec{v}_1 \cdot \vec{v}_1 \hat{n} \times \vec{S}_1 \cdot \vec{v}_2 + \frac{9}{8} \vec{v}_1 \cdot \vec{v}_2 \hat{n} \times \vec{S}_1 \cdot \vec{v}_1 \right) \right) \Bigg\}$$

{DiagSet[3, 9, 23],

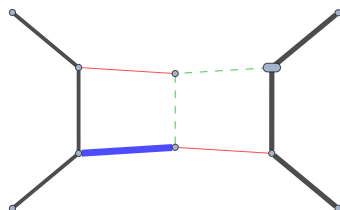

,

$$\frac{1}{r^4} G^3 m_1 m_2^2 \left( 19 \left( \hat{n} \cdot \vec{v}_2 \right)^2 \hat{n} \times \vec{S}_1 \cdot \vec{v}_1 - 33 \left( \hat{n} \cdot \vec{v}_2 \right)^2 \hat{n} \times \vec{S}_1 \cdot \vec{v}_2 + 4 \hat{n} \cdot \vec{v}_2 \vec{S}_1 \times \vec{v}_1 \cdot \vec{v}_2 + 14 \hat{n} \cdot \vec{v}_1 \hat{n} \cdot \vec{v}_2 \hat{n} \times \vec{S}_1 \cdot \vec{v}_2 - 6 \vec{v}_1 \cdot \vec{v}_2 \hat{n} \times \vec{S}_1 \cdot \vec{v}_2 - 3 \vec{v}_2 \cdot \vec{v}_2 \hat{n} \times \vec{S}_1 \cdot \vec{v}_1 + 9 \vec{v}_2 \cdot \vec{v}_2 \hat{n} \times \vec{S}_1 \cdot \vec{v}_2 + \pi^2 \left( - \frac{15}{16} \left( \hat{n} \cdot \vec{v}_2 \right)^2 \hat{n} \times \vec{S}_1 \cdot \vec{v}_1 + \frac{105}{16} \left( \hat{n} \cdot \vec{v}_2 \right)^2 \hat{n} \times \vec{S}_1 \cdot \vec{v}_2 - \frac{3}{4} \hat{n} \cdot \vec{v}_2 \vec{S}_1 \times \vec{v}_1 \cdot \vec{v}_2 - \frac{45}{8} \hat{n} \cdot \vec{v}_1 \hat{n} \cdot \vec{v}_2 \hat{n} \times \vec{S}_1 \cdot \vec{v}_2 + \frac{9}{8} \vec{v}_1 \cdot \vec{v}_2 \hat{n} \times \vec{S}_1 \cdot \vec{v}_2 + \frac{3}{16} \vec{v}_2 \cdot \vec{v}_2 \hat{n} \times \vec{S}_1 \cdot \vec{v}_1 - \frac{21}{16} \vec{v}_2 \cdot \vec{v}_2 \hat{n} \times \vec{S}_1 \cdot \vec{v}_2 \right) \right) + \frac{3 \pi^2 G^3 m_1 m_2^2 \hat{n} \cdot \vec{v}_2 \hat{n} \times \vec{S}_1 \cdot \vec{v}_2}{2 r^3} \Bigg\}$$

{DiagSet[3, 9, 24],

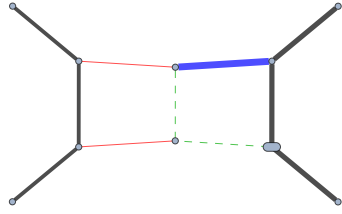

,

$$\frac{1}{r^4} G^3 m_1 m_2^2 \left( 147 (\hat{n} \cdot \vec{v}_1)^2 \hat{n} \times \vec{S}_1 \cdot \vec{v}_1 - (\hat{n} \cdot \vec{v}_1)^2 \hat{n} \times \vec{S}_1 \cdot \vec{v}_2 + 28 \hat{n} \cdot \vec{v}_1 \vec{S}_1 \times \vec{v}_1 \cdot \vec{v}_2 - \right. \\ \left. 146 \hat{n} \cdot \vec{v}_2 \hat{n} \cdot \vec{v}_1 \hat{n} \times \vec{S}_1 \cdot \vec{v}_1 - 27 \vec{v}_1 \cdot \vec{v}_1 \hat{n} \times \vec{S}_1 \cdot \vec{v}_1 - 3 \vec{v}_1 \cdot \vec{v}_1 \hat{n} \times \vec{S}_1 \cdot \vec{v}_2 + 30 \vec{v}_1 \cdot \vec{v}_2 \hat{n} \times \vec{S}_1 \cdot \vec{v}_1 + \right. \\ \left. \pi^2 \left( -\frac{15}{16} (\hat{n} \cdot \vec{v}_1)^2 \hat{n} \times \vec{S}_1 \cdot \vec{v}_1 - \frac{15}{16} (\hat{n} \cdot \vec{v}_1)^2 \hat{n} \times \vec{S}_1 \cdot \vec{v}_2 - \frac{3}{4} \hat{n} \cdot \vec{v}_1 \vec{S}_1 \times \vec{v}_1 \cdot \vec{v}_2 + \frac{15}{8} \hat{n} \cdot \vec{v}_2 \hat{n} \cdot \vec{v}_1 \hat{n} \times \vec{S}_1 \cdot \vec{v}_1 + \right. \right. \\ \left. \left. \frac{3}{16} \vec{v}_1 \cdot \vec{v}_1 \hat{n} \times \vec{S}_1 \cdot \vec{v}_1 + \frac{3}{16} \vec{v}_1 \cdot \vec{v}_1 \hat{n} \times \vec{S}_1 \cdot \vec{v}_2 - \frac{3}{8} \vec{v}_1 \cdot \vec{v}_2 \hat{n} \times \vec{S}_1 \cdot \vec{v}_1 \right) \right) - \frac{36 G^3 m_1 m_2^2 \hat{n} \cdot \vec{v}_1 \hat{n} \times \vec{S}_1 \cdot \vec{v}_1}{r^3} \Bigg\}$$

{DiagSet[3, 9, 25],

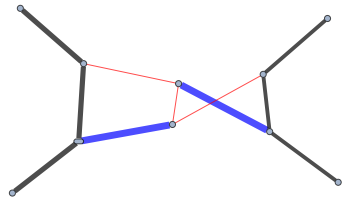

,  $\frac{1}{r^4}$

$$G^3 m_1 m_2^2 \left( -2 (\hat{n} \cdot \vec{v}_2)^2 \hat{n} \times \vec{S}_1 \cdot \vec{v}_1 + 4 \hat{n} \cdot \vec{v}_2 \vec{S}_1 \times \vec{v}_1 \cdot \vec{v}_2 + 21 \hat{n} \cdot \vec{v}_1 \hat{n} \cdot \vec{v}_2 \hat{n} \times \vec{S}_1 \cdot \vec{v}_2 - 4 \vec{v}_1 \cdot \vec{v}_2 \hat{n} \times \vec{S}_1 \cdot \vec{v}_2 + \right. \\ \left. \pi^2 \left( -\frac{3}{4} \hat{n} \cdot \vec{v}_2 \vec{S}_1 \times \vec{v}_1 \cdot \vec{v}_2 - \frac{15}{4} \hat{n} \cdot \vec{v}_1 \hat{n} \cdot \vec{v}_2 \hat{n} \times \vec{S}_1 \cdot \vec{v}_2 + \frac{3}{4} \vec{v}_1 \cdot \vec{v}_2 \hat{n} \times \vec{S}_1 \cdot \vec{v}_2 \right) + \vec{v}_2 \cdot \vec{v}_2 \hat{n} \times \vec{S}_1 \cdot \vec{v}_1 \right) \Bigg\}$$

{DiagSet[3, 9, 26],

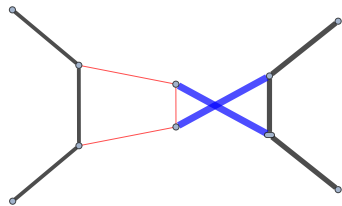

,  $\frac{1}{r^4}$

$$G^3 m_1 m_2^2 \left( \frac{7}{2} (\hat{n} \cdot \vec{v}_1)^2 \hat{n} \times \vec{S}_1 \cdot \vec{v}_1 - \frac{3}{2} \vec{v}_1 \cdot \vec{v}_1 \hat{n} \times \vec{S}_1 \cdot \vec{v}_1 + \pi^2 \left( \frac{3}{32} \vec{v}_1 \cdot \vec{v}_1 \hat{n} \times \vec{S}_1 \cdot \vec{v}_1 - \frac{15}{32} (\hat{n} \cdot \vec{v}_1)^2 \hat{n} \times \vec{S}_1 \cdot \vec{v}_1 \right) \right) \Bigg\}$$

{DiagSet[3, 9, 27],

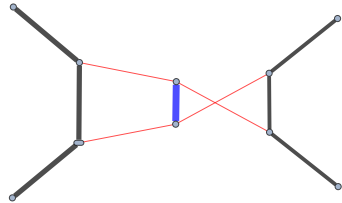

,

$$\frac{1}{r^3} G^3 m_1 m_2^2 \left( -8 \hat{n} \cdot \vec{v}_2 \hat{n} \times \vec{a}_1 \cdot \vec{S}_1 + \pi^2 \left( \frac{3}{4} \hat{n} \cdot \vec{v}_2 \hat{n} \times \vec{a}_1 \cdot \vec{S}_1 - \frac{1}{4} \vec{a}_1 \times \vec{S}_1 \cdot \vec{v}_2 - \frac{3}{4} \hat{n} \cdot \vec{v}_2 \hat{n} \times \vec{S}_1 \cdot \vec{v}_1 + \frac{1}{4} \vec{S}_1 \times \vec{v}_1 \cdot \vec{v}_2 \right) + \right. \\ \left. 8 \vec{a}_1 \times \vec{S}_1 \cdot \vec{v}_1 + 4 \vec{a}_1 \times \vec{S}_1 \cdot \vec{v}_2 + 8 \hat{n} \cdot \vec{v}_2 \hat{n} \times \vec{S}_1 \cdot \vec{v}_1 - 4 \vec{S}_1 \times \vec{v}_1 \cdot \vec{v}_2 \right) + \frac{1}{r^4} \\ G^3 m_1 m_2^2 \left( 8 \hat{n} \cdot \vec{v}_1 \vec{S}_1 \times \vec{v}_1 \cdot \vec{v}_2 - 40 \hat{n} \cdot \vec{v}_2 \hat{n} \cdot \vec{v}_1 \hat{n} \times \vec{S}_1 \cdot \vec{v}_1 + 24 \vec{v}_1 \cdot \vec{v}_1 \hat{n} \times \vec{S}_1 \cdot \vec{v}_1 + 12 \vec{v}_1 \cdot \vec{v}_2 \hat{n} \times \vec{S}_1 \cdot \vec{v}_1 + \right. \\ \left. \pi^2 \left( -\frac{3}{4} \hat{n} \cdot \vec{v}_1 \vec{S}_1 \times \vec{v}_1 \cdot \vec{v}_2 + \frac{15}{4} \hat{n} \cdot \vec{v}_2 \hat{n} \cdot \vec{v}_1 \hat{n} \times \vec{S}_1 \cdot \vec{v}_1 - \frac{3}{4} \vec{v}_1 \cdot \vec{v}_2 \hat{n} \times \vec{S}_1 \cdot \vec{v}_1 \right) + 36 \vec{v}_2 \cdot \vec{v}_2 \hat{n} \times \vec{S}_1 \cdot \vec{v}_1 \right) \Bigg\}$$

{DiagSet[3, 9, 28],

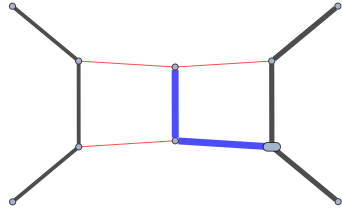

,

$$\frac{1}{r^3} \left( \frac{1}{\vec{S}_1 \times \vec{v}_1 \cdot \vec{v}_2} + \vec{S}_1 \times \vec{a}_1 \cdot \vec{v}_2 - \vec{S}_1 \times \vec{v}_1 \cdot \vec{a}_1 - 14 \hat{n} \times \vec{S}_1 \cdot \vec{v}_1 \hat{n} \cdot \vec{a}_1 + 19 \hat{n} \times \vec{S}_1 \cdot \vec{v}_2 \hat{n} \cdot \vec{a}_1 - \right. \\ \left. 31 \hat{n} \times \vec{S}_1 \cdot \vec{v}_1 \hat{n} \cdot \vec{v}_1 + 19 \hat{n} \times \vec{S}_1 \cdot \vec{v}_2 \hat{n} \cdot \vec{v}_1 - 17 \hat{n} \times \vec{S}_1 \cdot \vec{a}_1 \hat{n} \cdot \vec{v}_1 + 14 \hat{n} \times \vec{S}_1 \cdot \vec{v}_1 \hat{n} \cdot \vec{v}_2 + 14 \hat{n} \times \vec{S}_1 \cdot \vec{a}_1 \hat{n} \cdot \vec{v}_2 + \right. \\ \left. \pi^2 \left( -\frac{1}{4} \frac{1}{\vec{S}_1 \times \vec{v}_1 \cdot \vec{v}_2} - \frac{1}{4} \vec{S}_1 \times \vec{a}_1 \cdot \vec{v}_2 + \frac{1}{4} \vec{S}_1 \times \vec{v}_1 \cdot \vec{a}_1 + \frac{3}{8} \hat{n} \times \vec{S}_1 \cdot \vec{v}_1 \hat{n} \cdot \vec{a}_1 - \frac{3}{2} \hat{n} \times \vec{S}_1 \cdot \vec{v}_2 \hat{n} \cdot \vec{a}_1 + \frac{3}{2} \hat{n} \times \vec{S}_1 \cdot \vec{v}_1 \hat{n} \cdot \vec{v}_1 - \right. \right. \\ \left. \left. \frac{3}{2} \hat{n} \times \vec{S}_1 \cdot \vec{v}_2 \hat{n} \cdot \vec{v}_1 + \frac{9}{8} \hat{n} \times \vec{S}_1 \cdot \vec{a}_1 \hat{n} \cdot \vec{v}_1 - \frac{3}{4} \hat{n} \times \vec{S}_1 \cdot \vec{v}_1 \hat{n} \cdot \vec{v}_2 - \frac{3}{4} \hat{n} \times \vec{S}_1 \cdot \vec{a}_1 \hat{n} \cdot \vec{v}_2 \right) \right) m_1 m_2^2 G^3 + \frac{1}{r^4} \\ \left( -\frac{3}{4} \hat{n} \times \vec{S}_1 \cdot \vec{v}_1 (\hat{n} \cdot \vec{v}_1)^2 - \frac{115}{4} \hat{n} \times \vec{S}_1 \cdot \vec{v}_2 (\hat{n} \cdot \vec{v}_1)^2 - 16 \vec{S}_1 \times \vec{v}_1 \cdot \vec{v}_2 \hat{n} \cdot \vec{v}_1 + \frac{45}{2} \hat{n} \times \vec{S}_1 \cdot \vec{v}_1 \hat{n} \cdot \vec{v}_2 \hat{n} \cdot \vec{v}_1 + \right. \\ \left. \frac{15}{4} \hat{n} \times \vec{S}_1 \cdot \vec{v}_1 \vec{v}_1 \cdot \vec{v}_1 + \frac{15}{4} \hat{n} \times \vec{S}_1 \cdot \vec{v}_2 \vec{v}_1 \cdot \vec{v}_1 - \frac{17}{2} \hat{n} \times \vec{S}_1 \cdot \vec{v}_1 \vec{v}_1 \cdot \vec{v}_2 + \right. \\ \left. \pi^2 \left( -\frac{45}{64} \hat{n} \times \vec{S}_1 \cdot \vec{v}_1 (\hat{n} \cdot \vec{v}_1)^2 + \frac{135}{64} \hat{n} \times \vec{S}_1 \cdot \vec{v}_2 (\hat{n} \cdot \vec{v}_1)^2 + \frac{3}{4} \vec{S}_1 \times \vec{v}_1 \cdot \vec{v}_2 \hat{n} \cdot \vec{v}_1 + \frac{15}{32} \hat{n} \times \vec{S}_1 \cdot \vec{v}_1 \hat{n} \cdot \vec{v}_2 \hat{n} \cdot \vec{v}_1 + \right. \right. \\ \left. \left. \frac{9}{64} \hat{n} \times \vec{S}_1 \cdot \vec{v}_1 \vec{v}_1 \cdot \vec{v}_1 - \frac{27}{64} \hat{n} \times \vec{S}_1 \cdot \vec{v}_2 \vec{v}_1 \cdot \vec{v}_1 - \frac{3}{32} \hat{n} \times \vec{S}_1 \cdot \vec{v}_1 \vec{v}_1 \cdot \vec{v}_2 \right) \right) m_1 m_2^2 G^3 \Big\}$$

{DiagSet[3, 9, 29],

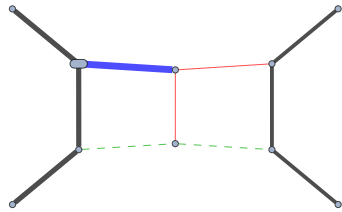

,  $\frac{1}{r^4}$

$$G^3 m_1 m_2^2 \left( -20 (\hat{n} \cdot \vec{v}_1)^2 \hat{n} \times \vec{S}_1 \cdot \vec{v}_2 - 8 \hat{n} \cdot \vec{v}_1 \vec{S}_1 \times \vec{v}_1 \cdot \vec{v}_2 + 20 \hat{n} \cdot \vec{v}_2 \hat{n} \cdot \vec{v}_1 \hat{n} \times \vec{S}_1 \cdot \vec{v}_1 + 12 \vec{v}_1 \cdot \vec{v}_2 \hat{n} \times \vec{S}_1 \cdot \vec{v}_1 \right) \Big\}$$

{DiagSet[3, 9, 30],

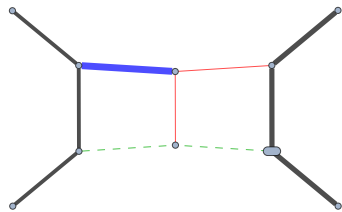

,  $\frac{1}{r^4}$

$$G^3 m_1 m_2^2 \left( 20 (\hat{n} \cdot \vec{v}_2)^2 \hat{n} \times \vec{S}_1 \cdot \vec{v}_2 + \pi^2 \left( \frac{3}{4} \vec{v}_2 \cdot \vec{v}_2 \hat{n} \times \vec{S}_1 \cdot \vec{v}_2 - \frac{15}{4} (\hat{n} \cdot \vec{v}_2)^2 \hat{n} \times \vec{S}_1 \cdot \vec{v}_2 \right) \right) \Big\}$$

{DiagSet[3, 9, 31],

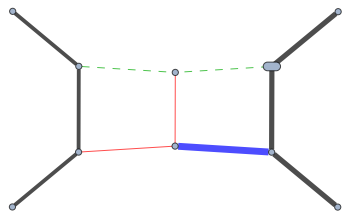

,  $\frac{1}{r^4}$

$$G^3 m_1 m_2^2 \left( 78 (\hat{n} \cdot \vec{v}_1)^2 \hat{n} \times \vec{S}_1 \cdot \vec{v}_2 + 36 \hat{n} \cdot \vec{v}_1 \vec{S}_1 \times \vec{v}_1 \cdot \vec{v}_2 - 64 \hat{n} \cdot \vec{v}_2 \hat{n} \cdot \vec{v}_1 \hat{n} \times \vec{S}_1 \cdot \vec{v}_1 - \right. \\ \left. 22 \vec{v}_1 \cdot \vec{v}_1 \hat{n} \times \vec{S}_1 \cdot \vec{v}_2 + 12 \vec{v}_1 \cdot \vec{v}_2 \hat{n} \times \vec{S}_1 \cdot \vec{v}_1 + \pi^2 \left( -\frac{75}{8} (\hat{n} \cdot \vec{v}_1)^2 \hat{n} \times \vec{S}_1 \cdot \vec{v}_2 - \right. \right. \\ \left. \left. \frac{15}{8} \vec{v}_1 \cdot \vec{v}_2 \hat{n} \times \vec{S}_1 \cdot \vec{v}_2 + \frac{15}{8} (\hat{n} \cdot \vec{v}_2)^2 \hat{n} \times \vec{S}_1 \cdot \vec{v}_2 \right) \right) \Big\}$$

$$6 \hat{n} \cdot \vec{v}_1 \vec{S}_1 \times \vec{v}_1 \cdot \vec{v}_2 + \frac{45}{4} \hat{n} \cdot \vec{v}_2 \hat{n} \cdot \vec{v}_1 \hat{n} \times \vec{S}_1 \cdot \vec{v}_1 + \frac{15}{8} \vec{v}_1 \cdot \vec{v}_1 \hat{n} \times \vec{S}_1 \cdot \vec{v}_2 - \frac{9}{4} \vec{v}_1 \cdot \vec{v}_2 \hat{n} \times \vec{S}_1 \cdot \vec{v}_1 \Big) \Big) \Big\}$$

$$\left\{ \text{DiagSet}[3, 9, 32], \frac{1}{r^4} \right\}$$
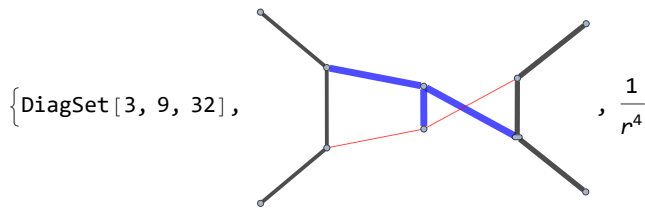

$$G^3 m_1 m_2^2 \left( \frac{87}{4} (\hat{n} \cdot \vec{v}_2)^2 \hat{n} \times \vec{S}_1 \cdot \vec{v}_1 - 8 \hat{n} \cdot \vec{v}_2 \vec{S}_1 \times \vec{v}_1 \cdot \vec{v}_2 - \frac{65}{2} \hat{n} \cdot \vec{v}_1 \hat{n} \cdot \vec{v}_2 \hat{n} \times \vec{S}_1 \cdot \vec{v}_2 + \right. \\ \left. \frac{49}{2} \vec{v}_1 \cdot \vec{v}_2 \hat{n} \times \vec{S}_1 \cdot \vec{v}_2 - \frac{107}{4} \vec{v}_2 \cdot \vec{v}_2 \hat{n} \times \vec{S}_1 \cdot \vec{v}_1 + \pi^2 \left( \frac{105}{64} (\hat{n} \cdot \vec{v}_2)^2 \hat{n} \times \vec{S}_1 \cdot \vec{v}_1 - \right. \right. \\ \left. \left. \frac{3}{8} \hat{n} \cdot \vec{v}_2 \vec{S}_1 \times \vec{v}_1 \cdot \vec{v}_2 + \frac{45}{32} \hat{n} \cdot \vec{v}_1 \hat{n} \cdot \vec{v}_2 \hat{n} \times \vec{S}_1 \cdot \vec{v}_2 - \frac{9}{32} \vec{v}_1 \cdot \vec{v}_2 \hat{n} \times \vec{S}_1 \cdot \vec{v}_2 - \frac{21}{64} \vec{v}_2 \cdot \vec{v}_2 \hat{n} \times \vec{S}_1 \cdot \vec{v}_1 \right) \right) \Big\}$$

$$\left\{ \text{DiagSet}[3, 9, 33], \right\}$$
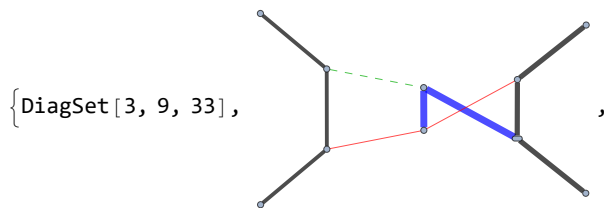

$$\frac{1}{r^3} \left( 17 \vec{S}_1 \times \vec{v}_1 \cdot \vec{v}_2 + 17 \vec{S}_1 \times \vec{a}_1 \cdot \vec{v}_2 + 21 \vec{S}_1 \times \vec{v}_1 \cdot \vec{a}_2 + 15 \hat{n} \times \vec{S}_1 \cdot \vec{v}_2 \hat{n} \cdot \vec{a}_1 - 16 \hat{n} \times \vec{S}_1 \cdot \vec{v}_1 \hat{n} \cdot \vec{a}_2 + \right. \\ \left. 15 \hat{n} \times \vec{S}_1 \cdot \vec{v}_2 \hat{n} \cdot \vec{v}_1 + 27 \hat{n} \times \vec{S}_1 \cdot \vec{a}_2 \hat{n} \cdot \vec{v}_1 + \pi^2 \left( -\frac{1}{4} \vec{S}_1 \times \vec{v}_1 \cdot \vec{v}_2 - \frac{1}{4} \vec{S}_1 \times \vec{a}_1 \cdot \vec{v}_2 - \frac{5}{4} \vec{S}_1 \times \vec{v}_1 \cdot \vec{a}_2 - \right. \right. \\ \left. \left. \frac{3}{4} \hat{n} \times \vec{S}_1 \cdot \vec{v}_2 \hat{n} \cdot \vec{a}_1 + \frac{3}{2} \hat{n} \times \vec{S}_1 \cdot \vec{v}_1 \hat{n} \cdot \vec{a}_2 - \frac{3}{4} \hat{n} \times \vec{S}_1 \cdot \vec{v}_2 \hat{n} \cdot \vec{v}_1 - \frac{9}{4} \hat{n} \times \vec{S}_1 \cdot \vec{a}_2 \hat{n} \cdot \vec{v}_1 \right) \right) m_1 m_2^2 G^3 + \frac{1}{r^4} \\ \left( -91 \hat{n} \times \vec{S}_1 \cdot \vec{v}_2 (\hat{n} \cdot \vec{v}_1)^2 - 64 \vec{S}_1 \times \vec{v}_1 \cdot \vec{v}_2 \hat{n} \cdot \vec{v}_1 + 52 \hat{n} \times \vec{S}_1 \cdot \vec{v}_1 \hat{n} \cdot \vec{v}_2 \hat{n} \cdot \vec{v}_1 + 163 \hat{n} \times \vec{S}_1 \cdot \vec{v}_2 \hat{n} \cdot \vec{v}_2 \hat{n} \cdot \vec{v}_1 - \right. \\ \left. \frac{177}{2} \hat{n} \times \vec{S}_1 \cdot \vec{v}_1 (\hat{n} \cdot \vec{v}_2)^2 + 78 \vec{S}_1 \times \vec{v}_1 \cdot \vec{v}_2 \hat{n} \cdot \vec{v}_2 + 21 \hat{n} \times \vec{S}_1 \cdot \vec{v}_2 \vec{v}_1 \cdot \vec{v}_1 - 14 \hat{n} \times \vec{S}_1 \cdot \vec{v}_1 \vec{v}_1 \cdot \vec{v}_2 - \right. \\ \left. 39 \hat{n} \times \vec{S}_1 \cdot \vec{v}_2 \vec{v}_1 \cdot \vec{v}_2 + \frac{61}{2} \hat{n} \times \vec{S}_1 \cdot \vec{v}_1 \vec{v}_2 \cdot \vec{v}_2 + \pi^2 \left( \frac{75}{8} \hat{n} \times \vec{S}_1 \cdot \vec{v}_2 (\hat{n} \cdot \vec{v}_1)^2 + \frac{21}{4} \vec{S}_1 \times \vec{v}_1 \cdot \vec{v}_2 \hat{n} \cdot \vec{v}_1 - \right. \right. \\ \left. \left. \frac{15}{2} \hat{n} \times \vec{S}_1 \cdot \vec{v}_1 \hat{n} \cdot \vec{v}_2 \hat{n} \cdot \vec{v}_1 - \frac{255}{16} \hat{n} \times \vec{S}_1 \cdot \vec{v}_2 \hat{n} \cdot \vec{v}_2 \hat{n} \cdot \vec{v}_1 + \frac{225}{32} \hat{n} \times \vec{S}_1 \cdot \vec{v}_1 (\hat{n} \cdot \vec{v}_2)^2 - 6 \vec{S}_1 \times \vec{v}_1 \cdot \vec{v}_2 \hat{n} \cdot \vec{v}_2 - \right. \right. \\ \left. \left. \frac{15}{8} \hat{n} \times \vec{S}_1 \cdot \vec{v}_2 \vec{v}_1 \cdot \vec{v}_1 + \frac{3}{2} \hat{n} \times \vec{S}_1 \cdot \vec{v}_1 \vec{v}_1 \cdot \vec{v}_2 + \frac{51}{16} \hat{n} \times \vec{S}_1 \cdot \vec{v}_2 \vec{v}_1 \cdot \vec{v}_2 - \frac{45}{32} \hat{n} \times \vec{S}_1 \cdot \vec{v}_1 \vec{v}_2 \cdot \vec{v}_2 \right) \right) m_1 m_2^2 G^3 \Big\}$$

$$\left\{ \text{DiagSet}[3, 9, 34], \right\}$$
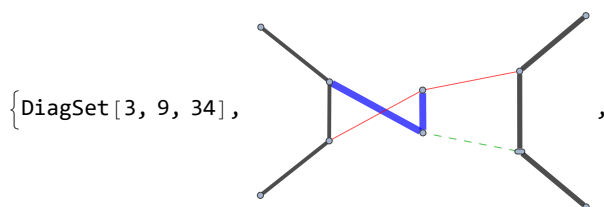

$$\frac{1}{r^3} G^3 m_1 m_2^2 \left( 3 \hat{n} \cdot \vec{a}_2 \hat{n} \times \vec{S}_1 \cdot \vec{v}_2 + 3 \hat{n} \cdot \vec{v}_2 \hat{n} \times \vec{S}_1 \cdot \vec{a}_2 + \pi^2 \left( -\frac{3}{4} \hat{n} \cdot \vec{a}_2 \hat{n} \times \vec{S}_1 \cdot \vec{v}_2 - \frac{3}{4} \hat{n} \cdot \vec{v}_2 \hat{n} \times \vec{S}_1 \cdot \vec{a}_2 \right) + 5 \hat{n} \cdot \vec{v}_2 \hat{n} \times \vec{S}_1 \cdot \vec{v}_2 \right) + \\ \frac{1}{r^4} G^3 m_1 m_2^2 \left( 34 (\hat{n} \cdot \vec{v}_2)^2 \hat{n} \times \vec{S}_1 \cdot \vec{v}_1 + \frac{29}{4} (\hat{n} \cdot \vec{v}_2)^2 \hat{n} \times \vec{S}_1 \cdot \vec{v}_2 - 27 \hat{n} \cdot \vec{v}_2 \vec{S}_1 \times \vec{v}_1 \cdot \vec{v}_2 - \right. \\ \left. 41 \hat{n} \cdot \vec{v}_1 \hat{n} \cdot \vec{v}_2 \hat{n} \times \vec{S}_1 \cdot \vec{v}_2 + 7 \vec{v}_1 \cdot \vec{v}_2 \hat{n} \times \vec{S}_1 \cdot \vec{v}_2 + 8 \vec{v}_2 \cdot \vec{v}_2 \hat{n} \times \vec{S}_1 \cdot \vec{v}_1 - \frac{49}{4} \vec{v}_2 \cdot \vec{v}_2 \hat{n} \times \vec{S}_1 \cdot \vec{v}_2 + \right.$$

$$\pi^2 \left( -\frac{15}{8} (\hat{n} \cdot \vec{v}_2)^2 \hat{n} \times \vec{S}_1 \cdot \vec{v}_1 + \frac{15}{64} (\hat{n} \cdot \vec{v}_2)^2 \hat{n} \times \vec{S}_1 \cdot \vec{v}_2 + \frac{9}{8} \hat{n} \cdot \vec{v}_2 \vec{S}_1 \times \vec{v}_1 \cdot \vec{v}_2 + \frac{15}{8} \hat{n} \cdot \vec{v}_1 \hat{n} \cdot \vec{v}_2 \hat{n} \times \vec{S}_1 \cdot \vec{v}_2 - \frac{3}{8} \vec{v}_1 \cdot \vec{v}_2 \hat{n} \times \vec{S}_1 \cdot \vec{v}_2 + \frac{3}{8} \vec{v}_2 \cdot \vec{v}_2 \hat{n} \times \vec{S}_1 \cdot \vec{v}_1 - \frac{3}{64} \vec{v}_2 \cdot \vec{v}_2 \hat{n} \times \vec{S}_1 \cdot \vec{v}_2 \right) \Bigg\}$$

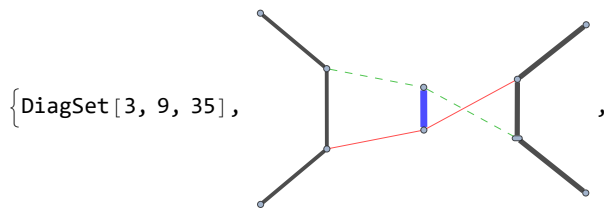

$$\frac{\left( 5 \hat{n} \times \vec{S}_1 \cdot \vec{a}_2 - \frac{1}{4} \pi^2 \hat{n} \times \vec{S}_1 \cdot \vec{a}_2 \right) m_1 m_2^2 G^3}{r^2} + \frac{1}{r^3} \left( 32 \vec{S}_1 \times \vec{v}_1 \cdot \vec{v}_2 + 32 \vec{S}_1 \times \vec{a}_1 \cdot \vec{v}_2 - 5 \vec{S}_1 \times \vec{v}_1 \cdot \vec{a}_2 + 14 \hat{n} \times \vec{S}_1 \cdot \vec{v}_1 \hat{n} \cdot \vec{a}_2 - 5 \hat{n} \times \vec{S}_1 \cdot \vec{a}_2 \hat{n} \cdot \vec{v}_1 - 32 \hat{n} \times \vec{S}_1 \cdot \vec{v}_1 \hat{n} \cdot \vec{v}_2 - 8 \hat{n} \times \vec{S}_1 \cdot \vec{v}_2 \hat{n} \cdot \vec{v}_2 - 32 \hat{n} \times \vec{S}_1 \cdot \vec{a}_1 \hat{n} \cdot \vec{v}_2 + \pi^2 \left( -\left( \vec{S}_1 \times \vec{v}_1 \cdot \vec{v}_2 \right) - \vec{S}_1 \times \vec{a}_1 \cdot \vec{v}_2 + \frac{1}{8} \vec{S}_1 \times \vec{v}_1 \cdot \vec{a}_2 - \frac{3}{8} \hat{n} \times \vec{S}_1 \cdot \vec{v}_1 \hat{n} \cdot \vec{a}_2 + 3 \hat{n} \times \vec{S}_1 \cdot \vec{v}_1 \hat{n} \cdot \vec{v}_2 + \frac{3}{4} \hat{n} \times \vec{S}_1 \cdot \vec{v}_2 \hat{n} \cdot \vec{v}_2 + 3 \hat{n} \times \vec{S}_1 \cdot \vec{a}_1 \hat{n} \cdot \vec{v}_2 \right) \right) m_1 m_2^2 G^3 + \frac{1}{r^4} \left( \frac{77}{2} \hat{n} \times \vec{S}_1 \cdot \vec{v}_1 (\hat{n} \cdot \vec{v}_2)^2 - 17 \vec{S}_1 \times \vec{v}_1 \cdot \vec{v}_2 \hat{n} \cdot \vec{v}_2 + 48 \hat{n} \times \vec{S}_1 \cdot \vec{v}_1 \hat{n} \cdot \vec{v}_1 \hat{n} \cdot \vec{v}_2 - 22 \hat{n} \times \vec{S}_1 \cdot \vec{v}_2 \hat{n} \cdot \vec{v}_1 \hat{n} \cdot \vec{v}_2 - 20 \vec{S}_1 \times \vec{v}_1 \cdot \vec{v}_2 \hat{n} \cdot \vec{v}_1 - 24 \hat{n} \times \vec{S}_1 \cdot \vec{v}_2 \vec{v}_1 \cdot \vec{v}_1 - 36 \hat{n} \times \vec{S}_1 \cdot \vec{v}_1 \vec{v}_1 \cdot \vec{v}_2 + 8 \hat{n} \times \vec{S}_1 \cdot \vec{v}_2 \vec{v}_1 \cdot \vec{v}_2 - \frac{9}{2} \hat{n} \times \vec{S}_1 \cdot \vec{v}_1 \vec{v}_2 \cdot \vec{v}_2 - 32 \hat{n} \times \vec{S}_1 \cdot \vec{v}_2 \vec{v}_2 \cdot \vec{v}_2 + \pi^2 \left( -\frac{75}{32} \hat{n} \times \vec{S}_1 \cdot \vec{v}_1 (\hat{n} \cdot \vec{v}_2)^2 + \frac{9}{8} \vec{S}_1 \times \vec{v}_1 \cdot \vec{v}_2 \hat{n} \cdot \vec{v}_2 - \frac{15}{4} \hat{n} \times \vec{S}_1 \cdot \vec{v}_1 \hat{n} \cdot \vec{v}_1 \hat{n} \cdot \vec{v}_2 + \frac{15}{16} \hat{n} \times \vec{S}_1 \cdot \vec{v}_2 \hat{n} \cdot \vec{v}_1 \hat{n} \cdot \vec{v}_2 + \frac{3}{4} \vec{S}_1 \times \vec{v}_1 \cdot \vec{v}_2 \hat{n} \cdot \vec{v}_1 + \frac{3}{4} \hat{n} \times \vec{S}_1 \cdot \vec{v}_1 \vec{v}_1 \cdot \vec{v}_2 - \frac{3}{16} \hat{n} \times \vec{S}_1 \cdot \vec{v}_2 \vec{v}_1 \cdot \vec{v}_2 + \frac{15}{32} \hat{n} \times \vec{S}_1 \cdot \vec{v}_1 \vec{v}_2 \cdot \vec{v}_2 \right) \right) m_1 m_2^2 G^3 \Bigg\}$$

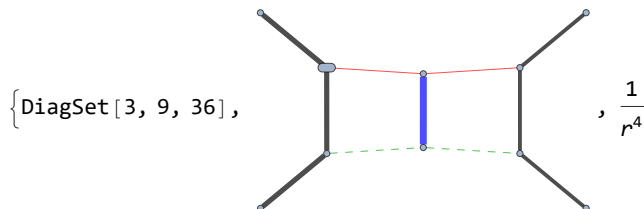

$$G^3 m_1 m_2^2 \left( -40 \hat{n} \cdot \vec{v}_1 \vec{S}_1 \times \vec{v}_1 \cdot \vec{v}_2 + 224 \hat{n} \cdot \vec{v}_2 \hat{n} \cdot \vec{v}_1 \hat{n} \times \vec{S}_1 \cdot \vec{v}_1 - 104 \vec{v}_1 \cdot \vec{v}_2 \hat{n} \times \vec{S}_1 \cdot \vec{v}_1 + \pi^2 \left( \frac{9}{2} \hat{n} \cdot \vec{v}_1 \vec{S}_1 \times \vec{v}_1 \cdot \vec{v}_2 - \frac{45}{2} \hat{n} \cdot \vec{v}_2 \hat{n} \cdot \vec{v}_1 \hat{n} \times \vec{S}_1 \cdot \vec{v}_1 + \frac{9}{2} \vec{v}_1 \cdot \vec{v}_2 \hat{n} \times \vec{S}_1 \cdot \vec{v}_1 \right) \right) \Bigg\}$$

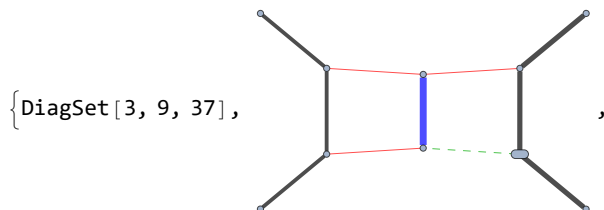

$$\frac{1}{r^2} \left( -64 \hat{n} \times \vec{S}_1 \cdot \vec{a}_1 - 32 \hat{n} \times \vec{S}_1 \cdot \vec{v}_1 - 32 \hat{n} \times \vec{S}_1 \cdot \vec{a}_1 + \pi^2 \left( 4 \hat{n} \times \vec{S}_1 \cdot \vec{a}_1 + 2 \hat{n} \times \vec{S}_1 \cdot \vec{v}_1 + 2 \hat{n} \times \vec{S}_1 \cdot \vec{a}_1 \right) \right) m_1 m_2^2 G^3 + \frac{1}{r^3} \left( 2 \vec{S}_1 \times \vec{v}_1 \cdot \vec{v}_2 + 2 \vec{S}_1 \times \vec{a}_1 \cdot \vec{v}_2 + 2 \vec{S}_1 \times \vec{v}_1 \cdot \vec{a}_1 + 22 \hat{n} \times \vec{S}_1 \cdot \vec{v}_1 \hat{n} \cdot \vec{a}_1 + 44 \hat{n} \times \vec{S}_1 \cdot \vec{v}_1 \hat{n} \cdot \vec{v}_1 + \hat{n} \times \vec{S}_1 \cdot \vec{v}_2 \hat{n} \cdot \vec{v}_1 + 44 \hat{n} \times \vec{S}_1 \cdot \vec{a}_1 \hat{n} \cdot \vec{v}_1 - 23 \hat{n} \times \vec{S}_1 \cdot \vec{v}_1 \hat{n} \cdot \vec{v}_2 - 22 \hat{n} \times \vec{S}_1 \cdot \vec{a}_1 \hat{n} \cdot \vec{v}_2 + \pi^2 \left( -\frac{1}{2} \vec{S}_1 \times \vec{v}_1 \cdot \vec{v}_2 - \frac{1}{2} \vec{S}_1 \times \vec{a}_1 \cdot \vec{v}_2 - \frac{1}{2} \vec{S}_1 \times \vec{v}_1 \cdot \vec{a}_1 - \right. \right.$$

$$\begin{aligned} & \left. \frac{3}{2} \hat{n} \times \vec{S}_1 \cdot \vec{v}_1 \hat{n} \cdot \vec{a}_1 - 3 \hat{n} \times \vec{S}_1 \cdot \vec{v}_1 \hat{n} \cdot \vec{v}_1 - 3 \hat{n} \times \vec{S}_1 \cdot \vec{a}_1 \hat{n} \cdot \vec{v}_1 + \frac{3}{2} \hat{n} \times \vec{S}_1 \cdot \vec{v}_1 \hat{n} \cdot \vec{v}_2 + \frac{3}{2} \hat{n} \times \vec{S}_1 \cdot \vec{a}_1 \hat{n} \cdot \vec{v}_2 \right) \Bigg) m_1 m_2^2 G^3 + \\ & \frac{1}{r^4} \left( -58 \hat{n} \times \vec{S}_1 \cdot \vec{v}_1 (\hat{n} \cdot \vec{v}_1)^2 - \frac{1}{4} \hat{n} \times \vec{S}_1 \cdot \vec{v}_2 (\hat{n} \cdot \vec{v}_1)^2 - 24 \vec{S}_1 \times \vec{v}_1 \cdot \vec{v}_2 \hat{n} \cdot \vec{v}_1 + \frac{177}{2} \hat{n} \times \vec{S}_1 \cdot \vec{v}_1 \hat{n} \cdot \vec{v}_2 \hat{n} \cdot \vec{v}_1 - \right. \\ & 10 \hat{n} \times \vec{S}_1 \cdot \vec{v}_1 \vec{v}_1 \cdot \vec{v}_1 + \frac{57}{4} \hat{n} \times \vec{S}_1 \cdot \vec{v}_2 \vec{v}_1 \cdot \vec{v}_1 - \frac{27}{2} \hat{n} \times \vec{S}_1 \cdot \vec{v}_1 \vec{v}_1 \cdot \vec{v}_2 + \pi^2 \\ & \left( \frac{15}{4} \hat{n} \times \vec{S}_1 \cdot \vec{v}_1 (\hat{n} \cdot \vec{v}_1)^2 - \frac{15}{64} \hat{n} \times \vec{S}_1 \cdot \vec{v}_2 (\hat{n} \cdot \vec{v}_1)^2 + \frac{3}{2} \vec{S}_1 \times \vec{v}_1 \cdot \vec{v}_2 \hat{n} \cdot \vec{v}_1 - \frac{255}{32} \hat{n} \times \vec{S}_1 \cdot \vec{v}_1 \hat{n} \cdot \vec{v}_2 \hat{n} \cdot \vec{v}_1 - \frac{3}{4} \hat{n} \times \vec{S}_1 \cdot \vec{v}_1 \right. \\ & \left. \vec{v}_1 \cdot \vec{v}_1 + \frac{3}{64} \hat{n} \times \vec{S}_1 \cdot \vec{v}_2 \vec{v}_1 \cdot \vec{v}_1 + \frac{51}{32} \hat{n} \times \vec{S}_1 \cdot \vec{v}_1 \vec{v}_1 \cdot \vec{v}_2 \right) - 36 \hat{n} \times \vec{S}_1 \cdot \vec{v}_1 \vec{v}_2 \cdot \vec{v}_2 + 30 \hat{n} \times \vec{S}_1 \cdot \vec{v}_2 \vec{v}_2 \cdot \vec{v}_2 \Bigg) m_1 m_2^2 G^3 \Bigg\} \end{aligned}$$

{DiagSet[3, 9, 38], 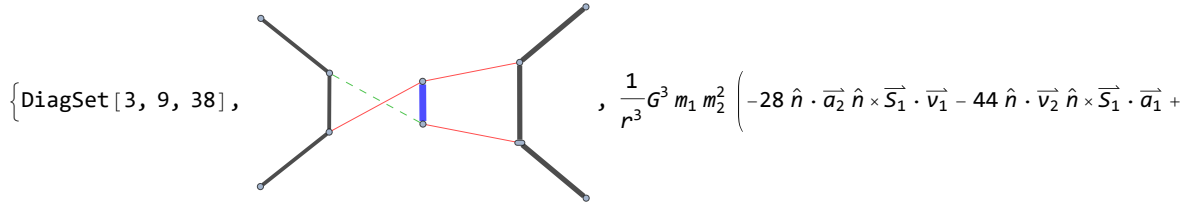 ,  $\frac{1}{r^3} G^3 m_1 m_2^2 \left( -28 \hat{n} \cdot \vec{a}_2 \hat{n} \times \vec{S}_1 \cdot \vec{v}_1 - 44 \hat{n} \cdot \vec{v}_2 \hat{n} \times \vec{S}_1 \cdot \vec{a}_1 + \right.$

$$\begin{aligned} & \pi^2 \left( 3 \hat{n} \cdot \vec{a}_2 \hat{n} \times \vec{S}_1 \cdot \vec{v}_1 + 3 \hat{n} \cdot \vec{v}_2 \hat{n} \times \vec{S}_1 \cdot \vec{a}_1 - \vec{S}_1 \times \vec{a}_1 \cdot \vec{v}_2 - \vec{S}_1 \times \vec{v}_1 \cdot \vec{a}_2 + 3 \hat{n} \cdot \vec{v}_2 \hat{n} \times \vec{S}_1 \cdot \vec{v}_1 - \left( \frac{1}{\vec{S}_1 \times \vec{v}_1 \cdot \vec{v}_2} \right) \right) + \\ & 4 \vec{S}_1 \times \vec{a}_1 \cdot \vec{v}_2 + 4 \vec{S}_1 \times \vec{v}_1 \cdot \vec{a}_2 - 44 \hat{n} \cdot \vec{v}_2 \hat{n} \times \vec{S}_1 \cdot \vec{v}_1 + 4 \frac{1}{\vec{S}_1 \times \vec{v}_1 \cdot \vec{v}_2} \Bigg) + \frac{1}{r^4} \\ & G^3 m_1 m_2^2 \left( -168 (\hat{n} \cdot \vec{v}_2)^2 \hat{n} \times \vec{S}_1 \cdot \vec{v}_1 + 72 \hat{n} \cdot \vec{v}_2 \vec{S}_1 \times \vec{v}_1 \cdot \vec{v}_2 + 116 \hat{n} \cdot \vec{v}_1 \hat{n} \cdot \vec{v}_2 \hat{n} \times \vec{S}_1 \cdot \vec{v}_1 - 4 \hat{n} \cdot \vec{v}_1 \vec{S}_1 \times \vec{v}_1 \cdot \vec{v}_2 - \right. \\ & 4 \vec{v}_1 \cdot \vec{v}_2 \hat{n} \times \vec{S}_1 \cdot \vec{v}_1 + 16 \vec{v}_2 \cdot \vec{v}_2 \hat{n} \times \vec{S}_1 \cdot \vec{v}_1 + \pi^2 \left( 15 (\hat{n} \cdot \vec{v}_2)^2 \hat{n} \times \vec{S}_1 \cdot \vec{v}_1 - 6 \hat{n} \cdot \vec{v}_2 \vec{S}_1 \times \vec{v}_1 \cdot \vec{v}_2 - \right. \\ & \left. \frac{15}{2} \hat{n} \cdot \vec{v}_1 \hat{n} \cdot \vec{v}_2 \hat{n} \times \vec{S}_1 \cdot \vec{v}_1 + \frac{3}{2} \hat{n} \cdot \vec{v}_1 \vec{S}_1 \times \vec{v}_1 \cdot \vec{v}_2 + \frac{3}{2} \vec{v}_1 \cdot \vec{v}_2 \hat{n} \times \vec{S}_1 \cdot \vec{v}_1 - 3 \vec{v}_2 \cdot \vec{v}_2 \hat{n} \times \vec{S}_1 \cdot \vec{v}_1 \right) \Bigg) \Bigg\} \end{aligned}$$

{DiagSet[3, 9, 39], 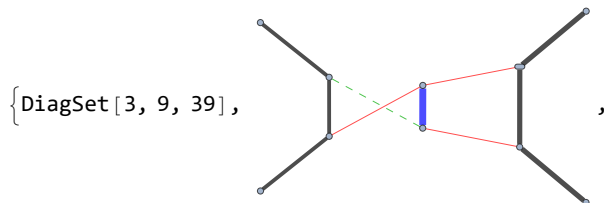 ,

$$\begin{aligned} & \frac{1}{r^3} G^3 m_1 m_2^2 \left( -164 \hat{n} \cdot \vec{a}_2 \hat{n} \times \vec{S}_1 \cdot \vec{v}_1 + \pi^2 \left( 9 \hat{n} \cdot \vec{a}_2 \hat{n} \times \vec{S}_1 \cdot \vec{v}_1 - 3 \vec{S}_1 \times \vec{v}_1 \cdot \vec{a}_2 \right) + 60 \vec{S}_1 \times \vec{v}_1 \cdot \vec{a}_2 \right) + \frac{1}{r^4} \\ & G^3 m_1 m_2^2 \left( -52 (\hat{n} \cdot \vec{v}_2)^2 \hat{n} \times \vec{S}_1 \cdot \vec{v}_1 + 16 \hat{n} \cdot \vec{v}_2 \vec{S}_1 \times \vec{v}_1 \cdot \vec{v}_2 + 104 \hat{n} \cdot \vec{v}_1 \hat{n} \cdot \vec{v}_2 \hat{n} \times \vec{S}_1 \cdot \vec{v}_1 - 40 \hat{n} \cdot \vec{v}_1 \vec{S}_1 \times \vec{v}_1 \cdot \vec{v}_2 - \right. \\ & 8 \vec{v}_1 \cdot \vec{v}_2 \hat{n} \times \vec{S}_1 \cdot \vec{v}_1 + \pi^2 \left( \frac{3}{2} \hat{n} \cdot \vec{v}_1 \vec{S}_1 \times \vec{v}_1 \cdot \vec{v}_2 - \frac{15}{2} \hat{n} \cdot \vec{v}_2 \hat{n} \cdot \vec{v}_1 \hat{n} \times \vec{S}_1 \cdot \vec{v}_1 + \frac{3}{2} \vec{v}_1 \cdot \vec{v}_2 \hat{n} \times \vec{S}_1 \cdot \vec{v}_1 \right) - 4 \vec{v}_2 \cdot \vec{v}_2 \hat{n} \times \vec{S}_1 \cdot \vec{v}_1 \Bigg) \Bigg\} \end{aligned}$$

{DiagSet[3, 9, 40], 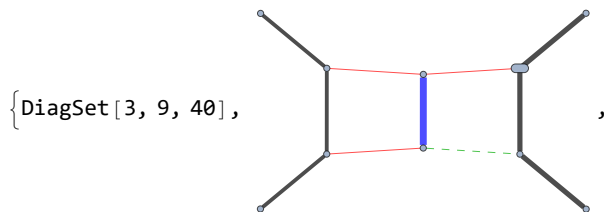 ,

$$\begin{aligned} & \frac{1}{r^3} G^3 m_1 m_2^2 \left( 148 \hat{n} \cdot \vec{a}_1 \hat{n} \times \vec{S}_1 \cdot \vec{v}_1 + \pi^2 \left( 3 \vec{S}_1 \times \vec{v}_1 \cdot \vec{a}_1 - 9 \hat{n} \cdot \vec{a}_1 \hat{n} \times \vec{S}_1 \cdot \vec{v}_1 \right) - 60 \vec{S}_1 \times \vec{v}_1 \cdot \vec{a}_1 \right) + \\ & \frac{1}{r^4} G^3 m_1 m_2^2 \left( -104 (\hat{n} \cdot \vec{v}_1)^2 \hat{n} \times \vec{S}_1 \cdot \vec{v}_1 + 12 \hat{n} \cdot \vec{v}_1 \vec{S}_1 \times \vec{v}_1 \cdot \vec{v}_2 + 52 \hat{n} \cdot \vec{v}_2 \hat{n} \cdot \vec{v}_1 \hat{n} \times \vec{S}_1 \cdot \vec{v}_1 + \right. \end{aligned}$$



$$8 \vec{v}_1 \cdot \vec{v}_1 \hat{n} \times \vec{S}_1 \cdot \vec{v}_1 + \pi^2 \left( \frac{15}{2} (\hat{n} \cdot \vec{v}_1)^2 \hat{n} \times \vec{S}_1 \cdot \vec{v}_1 - \frac{3}{2} \vec{v}_1 \cdot \vec{v}_1 \hat{n} \times \vec{S}_1 \cdot \vec{v}_1 \right) + 4 \vec{v}_1 \cdot \vec{v}_2 \hat{n} \times \vec{S}_1 \cdot \vec{v}_1 \Big) \Big\}$$

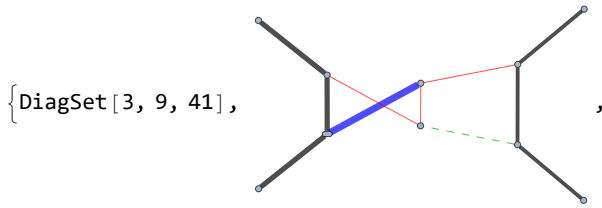

$$\begin{aligned} & \frac{1}{r^3} G^3 m_1 m_2^2 \left( -7 \hat{n} \cdot \vec{a}_1 \hat{n} \times \vec{S}_1 \cdot \vec{v}_2 + \pi^2 \left( \frac{9}{8} \hat{n} \cdot \vec{a}_1 \hat{n} \times \vec{S}_1 \cdot \vec{v}_2 + \frac{3}{8} \hat{n} \cdot \vec{v}_2 \hat{n} \times \vec{S}_1 \cdot \vec{a}_1 + \frac{1}{4} \vec{S}_1 \times \vec{a}_1 \cdot \vec{v}_2 + \frac{9}{8} \hat{n} \cdot \vec{v}_1 \hat{n} \times \vec{S}_1 \cdot \vec{v}_2 + \right. \right. \\ & \quad \left. \left. \frac{3}{8} \hat{n} \cdot \vec{v}_2 \hat{n} \times \vec{S}_1 \cdot \vec{v}_1 + \frac{1}{4} \vec{S}_1 \times \vec{v}_1 \cdot \vec{v}_2 \right) - \vec{S}_1 \times \vec{a}_1 \cdot \vec{v}_2 - 7 \hat{n} \cdot \vec{v}_1 \hat{n} \times \vec{S}_1 \cdot \vec{v}_2 - \left( \vec{S}_1 \times \vec{v}_1 \cdot \vec{v}_2 \right) \right) + \frac{1}{r^4} \\ & G^3 m_1 m_2^2 \left( \frac{39}{4} (\hat{n} \cdot \vec{v}_1)^2 \hat{n} \times \vec{S}_1 \cdot \vec{v}_2 + 7 \hat{n} \cdot \vec{v}_1 \vec{S}_1 \times \vec{v}_1 \cdot \vec{v}_2 - \frac{51}{2} \hat{n} \cdot \vec{v}_2 \hat{n} \cdot \vec{v}_1 \hat{n} \times \vec{S}_1 \cdot \vec{v}_1 - \frac{43}{2} \hat{n} \cdot \vec{v}_2 \hat{n} \cdot \vec{v}_1 \hat{n} \times \vec{S}_1 \cdot \vec{v}_2 - \right. \\ & \quad \left. \frac{3}{4} (\hat{n} \cdot \vec{v}_2)^2 \hat{n} \times \vec{S}_1 \cdot \vec{v}_1 - 3 \hat{n} \cdot \vec{v}_2 \vec{S}_1 \times \vec{v}_1 \cdot \vec{v}_2 - \frac{3}{4} \vec{v}_1 \cdot \vec{v}_1 \hat{n} \times \vec{S}_1 \cdot \vec{v}_2 + \frac{7}{2} \vec{v}_1 \cdot \vec{v}_2 \hat{n} \times \vec{S}_1 \cdot \vec{v}_1 + \right. \\ & \quad \left. \frac{5}{2} \vec{v}_1 \cdot \vec{v}_2 \hat{n} \times \vec{S}_1 \cdot \vec{v}_2 + \frac{3}{4} \vec{v}_2 \cdot \vec{v}_2 \hat{n} \times \vec{S}_1 \cdot \vec{v}_1 + \pi^2 \left( -\frac{75}{64} (\hat{n} \cdot \vec{v}_1)^2 \hat{n} \times \vec{S}_1 \cdot \vec{v}_2 - \frac{9}{8} \hat{n} \cdot \vec{v}_1 \vec{S}_1 \times \vec{v}_1 \cdot \vec{v}_2 + \right. \right. \\ & \quad \left. \left. \frac{105}{32} \hat{n} \cdot \vec{v}_2 \hat{n} \cdot \vec{v}_1 \hat{n} \times \vec{S}_1 \cdot \vec{v}_1 + \frac{135}{32} \hat{n} \cdot \vec{v}_2 \hat{n} \cdot \vec{v}_1 \hat{n} \times \vec{S}_1 \cdot \vec{v}_2 + \frac{75}{64} (\hat{n} \cdot \vec{v}_2)^2 \hat{n} \times \vec{S}_1 \cdot \vec{v}_1 + \frac{3}{8} \hat{n} \cdot \vec{v}_2 \vec{S}_1 \times \vec{v}_1 \cdot \vec{v}_2 + \right. \right. \\ & \quad \left. \left. \frac{15}{64} \vec{v}_1 \cdot \vec{v}_1 \hat{n} \times \vec{S}_1 \cdot \vec{v}_2 - \frac{21}{32} \vec{v}_1 \cdot \vec{v}_2 \hat{n} \times \vec{S}_1 \cdot \vec{v}_1 - \frac{27}{32} \vec{v}_1 \cdot \vec{v}_2 \hat{n} \times \vec{S}_1 \cdot \vec{v}_2 - \frac{15}{64} \vec{v}_2 \cdot \vec{v}_2 \hat{n} \times \vec{S}_1 \cdot \vec{v}_1 \right) \right) \Big\} \end{aligned}$$

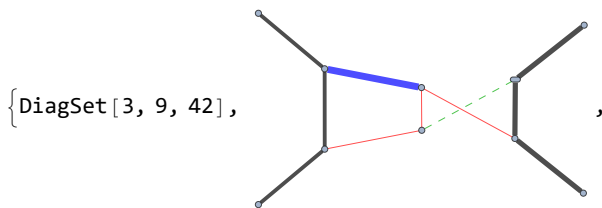

$$\begin{aligned} & \frac{1}{r^3} G^3 m_1 m_2^2 \left( 4 \hat{n} \cdot \vec{a}_2 \hat{n} \times \vec{S}_1 \cdot \vec{v}_2 - 4 \hat{n} \cdot \vec{v}_2 \hat{n} \times \vec{a}_2 \cdot \vec{S}_1 + \pi^2 \left( \frac{3}{4} \hat{n} \cdot \vec{v}_2 \hat{n} \times \vec{a}_2 \cdot \vec{S}_1 - \frac{3}{4} \hat{n} \cdot \vec{a}_2 \hat{n} \times \vec{S}_1 \cdot \vec{v}_2 \right) \right) + \frac{1}{r^4} \\ & G^3 m_1 m_2^2 \left( -7 (\hat{n} \cdot \vec{v}_2)^2 \hat{n} \times \vec{S}_1 \cdot \vec{v}_1 - 3 (\hat{n} \cdot \vec{v}_2)^2 \hat{n} \times \vec{S}_1 \cdot \vec{v}_2 - 9 \hat{n} \cdot \vec{v}_1 \hat{n} \cdot \vec{v}_2 \hat{n} \times \vec{S}_1 \cdot \vec{v}_2 + 2 \vec{v}_1 \cdot \vec{v}_2 \hat{n} \times \vec{S}_1 \cdot \vec{v}_2 + \right. \\ & \quad \left. 2 \vec{v}_2 \cdot \vec{v}_2 \hat{n} \times \vec{S}_1 \cdot \vec{v}_1 - \vec{v}_2 \cdot \vec{v}_2 \hat{n} \times \vec{S}_1 \cdot \vec{v}_2 + \pi^2 \left( \frac{15}{16} (\hat{n} \cdot \vec{v}_2)^2 \hat{n} \times \vec{S}_1 \cdot \vec{v}_1 + \frac{15}{16} (\hat{n} \cdot \vec{v}_2)^2 \hat{n} \times \vec{S}_1 \cdot \vec{v}_2 + \right. \right. \\ & \quad \left. \left. \frac{15}{8} \hat{n} \cdot \vec{v}_1 \hat{n} \cdot \vec{v}_2 \hat{n} \times \vec{S}_1 \cdot \vec{v}_2 - \frac{3}{8} \vec{v}_1 \cdot \vec{v}_2 \hat{n} \times \vec{S}_1 \cdot \vec{v}_2 - \frac{3}{16} \vec{v}_2 \cdot \vec{v}_2 \hat{n} \times \vec{S}_1 \cdot \vec{v}_1 - \frac{3}{16} \vec{v}_2 \cdot \vec{v}_2 \hat{n} \times \vec{S}_1 \cdot \vec{v}_2 \right) \right) \Big\} \end{aligned}$$

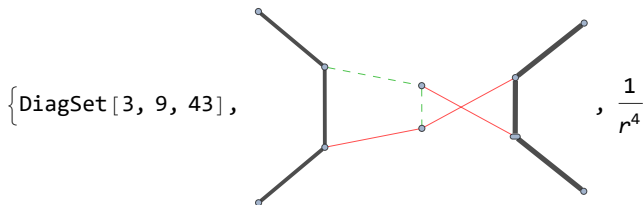

$$G^3 m_1 m_2^2 \left( 20 (\hat{n} \cdot \vec{v}_2)^2 \hat{n} \times \vec{S}_1 \cdot \vec{v}_1 + 8 \hat{n} \cdot \vec{v}_1 \vec{S}_1 \times \vec{v}_1 \cdot \vec{v}_2 - 8 \vec{v}_1 \cdot \vec{v}_2 \hat{n} \times \vec{S}_1 \cdot \vec{v}_1 + 4 \vec{v}_2 \cdot \vec{v}_2 \hat{n} \times \vec{S}_1 \cdot \vec{v}_1 \right) \Big\}$$

$\{\text{DiagSet}[3, 9, 44],$ 
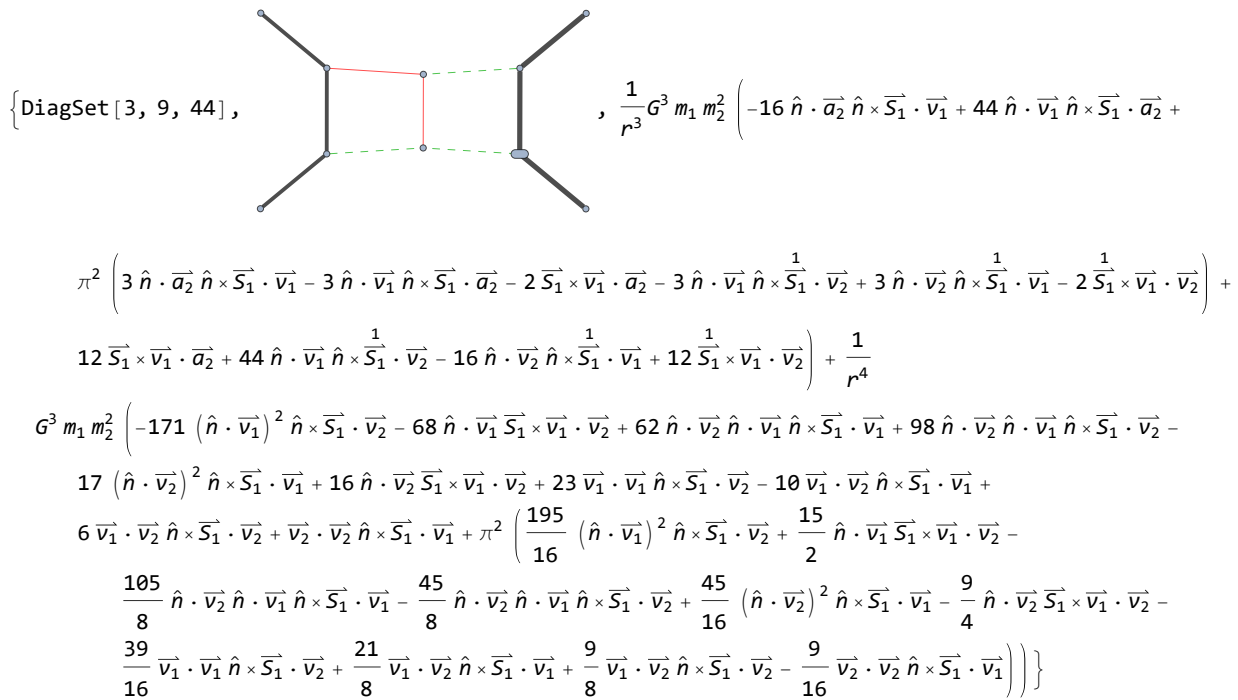
 $, \frac{1}{r^3} G^3 m_1 m_2^2 \left( -16 \hat{n} \cdot \vec{a}_2 \hat{n} \times \vec{S}_1 \cdot \vec{v}_1 + 44 \hat{n} \cdot \vec{v}_1 \hat{n} \times \vec{S}_1 \cdot \vec{a}_2 + \right.$ 
 $\pi^2 \left( 3 \hat{n} \cdot \vec{a}_2 \hat{n} \times \vec{S}_1 \cdot \vec{v}_1 - 3 \hat{n} \cdot \vec{v}_1 \hat{n} \times \vec{S}_1 \cdot \vec{a}_2 - 2 \vec{S}_1 \times \vec{v}_1 \cdot \vec{a}_2 - 3 \hat{n} \cdot \vec{v}_1 \hat{n} \times \vec{S}_1 \cdot \vec{v}_2 + 3 \hat{n} \cdot \vec{v}_2 \hat{n} \times \vec{S}_1 \cdot \vec{v}_1 - 2 \vec{S}_1 \times \vec{v}_1 \cdot \vec{v}_2 \right) +$ 
 $12 \vec{S}_1 \times \vec{v}_1 \cdot \vec{a}_2 + 44 \hat{n} \cdot \vec{v}_1 \hat{n} \times \vec{S}_1 \cdot \vec{v}_2 - 16 \hat{n} \cdot \vec{v}_2 \hat{n} \times \vec{S}_1 \cdot \vec{v}_1 + 12 \vec{S}_1 \times \vec{v}_1 \cdot \vec{v}_2 \Big) + \frac{1}{r^4}$ 
 $G^3 m_1 m_2^2 \left( -171 (\hat{n} \cdot \vec{v}_1)^2 \hat{n} \times \vec{S}_1 \cdot \vec{v}_2 - 68 \hat{n} \cdot \vec{v}_1 \vec{S}_1 \times \vec{v}_1 \cdot \vec{v}_2 + 62 \hat{n} \cdot \vec{v}_2 \hat{n} \cdot \vec{v}_1 \hat{n} \times \vec{S}_1 \cdot \vec{v}_1 + 98 \hat{n} \cdot \vec{v}_2 \hat{n} \cdot \vec{v}_1 \hat{n} \times \vec{S}_1 \cdot \vec{v}_2 - \right.$ 
 $17 (\hat{n} \cdot \vec{v}_2)^2 \hat{n} \times \vec{S}_1 \cdot \vec{v}_1 + 16 \hat{n} \cdot \vec{v}_2 \vec{S}_1 \times \vec{v}_1 \cdot \vec{v}_2 + 23 \vec{v}_1 \cdot \vec{v}_1 \hat{n} \times \vec{S}_1 \cdot \vec{v}_2 - 10 \vec{v}_1 \cdot \vec{v}_2 \hat{n} \times \vec{S}_1 \cdot \vec{v}_1 +$ 
 $6 \vec{v}_1 \cdot \vec{v}_2 \hat{n} \times \vec{S}_1 \cdot \vec{v}_2 + \vec{v}_2 \cdot \vec{v}_2 \hat{n} \times \vec{S}_1 \cdot \vec{v}_1 + \pi^2 \left( \frac{195}{16} (\hat{n} \cdot \vec{v}_1)^2 \hat{n} \times \vec{S}_1 \cdot \vec{v}_2 + \frac{15}{2} \hat{n} \cdot \vec{v}_1 \vec{S}_1 \times \vec{v}_1 \cdot \vec{v}_2 - \right.$ 
 $\frac{105}{8} \hat{n} \cdot \vec{v}_2 \hat{n} \cdot \vec{v}_1 \hat{n} \times \vec{S}_1 \cdot \vec{v}_1 - \frac{45}{8} \hat{n} \cdot \vec{v}_2 \hat{n} \cdot \vec{v}_1 \hat{n} \times \vec{S}_1 \cdot \vec{v}_2 + \frac{45}{16} (\hat{n} \cdot \vec{v}_2)^2 \hat{n} \times \vec{S}_1 \cdot \vec{v}_1 - \frac{9}{4} \hat{n} \cdot \vec{v}_2 \vec{S}_1 \times \vec{v}_1 \cdot \vec{v}_2 -$ 
 $\left. \frac{39}{16} \vec{v}_1 \cdot \vec{v}_1 \hat{n} \times \vec{S}_1 \cdot \vec{v}_2 + \frac{21}{8} \vec{v}_1 \cdot \vec{v}_2 \hat{n} \times \vec{S}_1 \cdot \vec{v}_1 + \frac{9}{8} \vec{v}_1 \cdot \vec{v}_2 \hat{n} \times \vec{S}_1 \cdot \vec{v}_2 - \frac{9}{16} \vec{v}_2 \cdot \vec{v}_2 \hat{n} \times \vec{S}_1 \cdot \vec{v}_1 \right) \Big) \Big\}$

$\{\text{DiagSet}[3, 9, 45],$ 
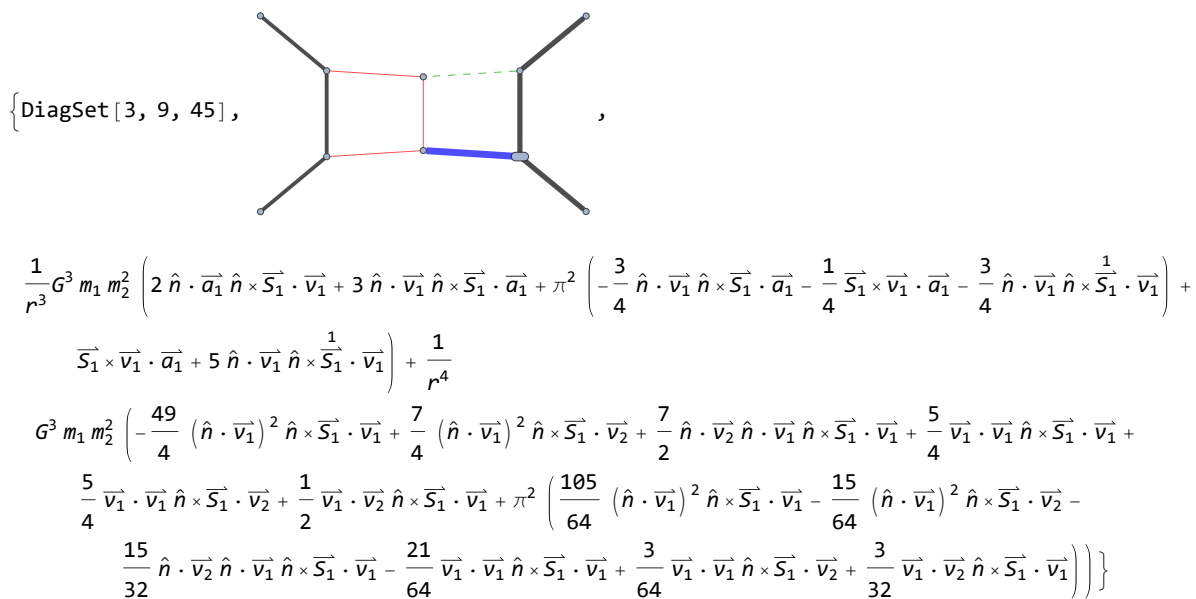
 $,$ 
 $\frac{1}{r^3} G^3 m_1 m_2^2 \left( 2 \hat{n} \cdot \vec{a}_1 \hat{n} \times \vec{S}_1 \cdot \vec{v}_1 + 3 \hat{n} \cdot \vec{v}_1 \hat{n} \times \vec{S}_1 \cdot \vec{a}_1 + \pi^2 \left( -\frac{3}{4} \hat{n} \cdot \vec{v}_1 \hat{n} \times \vec{S}_1 \cdot \vec{a}_1 - \frac{1}{4} \vec{S}_1 \times \vec{v}_1 \cdot \vec{a}_1 - \frac{3}{4} \hat{n} \cdot \vec{v}_1 \hat{n} \times \vec{S}_1 \cdot \vec{v}_1 \right) + \right.$ 
 $\left. \vec{S}_1 \times \vec{v}_1 \cdot \vec{a}_1 + 5 \hat{n} \cdot \vec{v}_1 \hat{n} \times \vec{S}_1 \cdot \vec{v}_1 \right) + \frac{1}{r^4}$ 
 $G^3 m_1 m_2^2 \left( -\frac{49}{4} (\hat{n} \cdot \vec{v}_1)^2 \hat{n} \times \vec{S}_1 \cdot \vec{v}_1 + \frac{7}{4} (\hat{n} \cdot \vec{v}_1)^2 \hat{n} \times \vec{S}_1 \cdot \vec{v}_2 + \frac{7}{2} \hat{n} \cdot \vec{v}_2 \hat{n} \cdot \vec{v}_1 \hat{n} \times \vec{S}_1 \cdot \vec{v}_1 + \frac{5}{4} \vec{v}_1 \cdot \vec{v}_1 \hat{n} \times \vec{S}_1 \cdot \vec{v}_1 + \right.$ 
 $\frac{5}{4} \vec{v}_1 \cdot \vec{v}_1 \hat{n} \times \vec{S}_1 \cdot \vec{v}_2 + \frac{1}{2} \vec{v}_1 \cdot \vec{v}_2 \hat{n} \times \vec{S}_1 \cdot \vec{v}_1 + \pi^2 \left( \frac{105}{64} (\hat{n} \cdot \vec{v}_1)^2 \hat{n} \times \vec{S}_1 \cdot \vec{v}_1 - \frac{15}{64} (\hat{n} \cdot \vec{v}_1)^2 \hat{n} \times \vec{S}_1 \cdot \vec{v}_2 - \right.$ 
 $\left. \frac{15}{32} \hat{n} \cdot \vec{v}_2 \hat{n} \cdot \vec{v}_1 \hat{n} \times \vec{S}_1 \cdot \vec{v}_1 - \frac{21}{64} \vec{v}_1 \cdot \vec{v}_1 \hat{n} \times \vec{S}_1 \cdot \vec{v}_1 + \frac{3}{64} \vec{v}_1 \cdot \vec{v}_1 \hat{n} \times \vec{S}_1 \cdot \vec{v}_2 + \frac{3}{32} \vec{v}_1 \cdot \vec{v}_2 \hat{n} \times \vec{S}_1 \cdot \vec{v}_1 \right) \Big) \Big\}$

$\{\text{DiagSet}[3, 9, 46],$ 
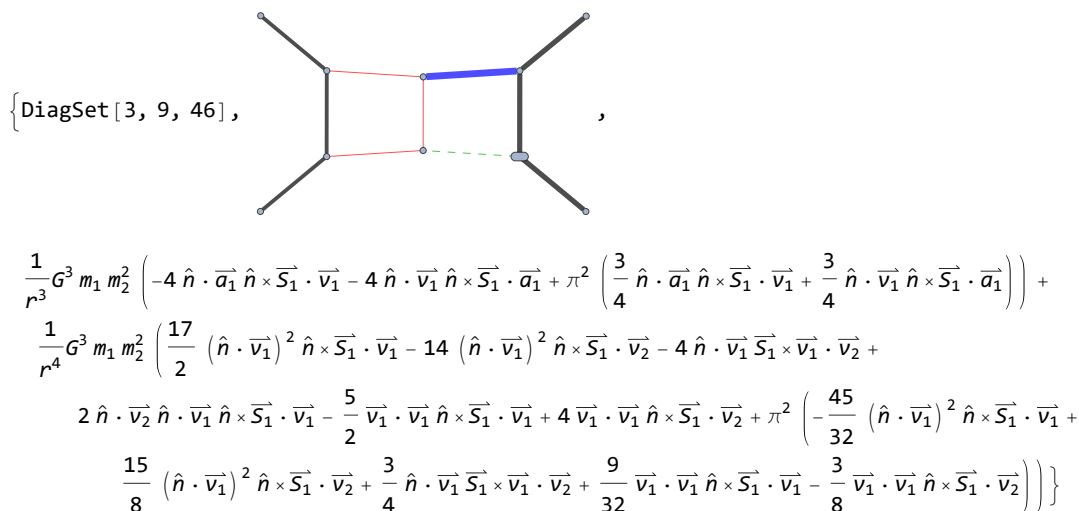
 $,$ 
 $\frac{1}{r^3} G^3 m_1 m_2^2 \left( -4 \hat{n} \cdot \vec{a}_1 \hat{n} \times \vec{S}_1 \cdot \vec{v}_1 - 4 \hat{n} \cdot \vec{v}_1 \hat{n} \times \vec{S}_1 \cdot \vec{a}_1 + \pi^2 \left( \frac{3}{4} \hat{n} \cdot \vec{a}_1 \hat{n} \times \vec{S}_1 \cdot \vec{v}_1 + \frac{3}{4} \hat{n} \cdot \vec{v}_1 \hat{n} \times \vec{S}_1 \cdot \vec{a}_1 \right) \right) +$ 
 $\frac{1}{r^4} G^3 m_1 m_2^2 \left( \frac{17}{2} (\hat{n} \cdot \vec{v}_1)^2 \hat{n} \times \vec{S}_1 \cdot \vec{v}_1 - 14 (\hat{n} \cdot \vec{v}_1)^2 \hat{n} \times \vec{S}_1 \cdot \vec{v}_2 - 4 \hat{n} \cdot \vec{v}_1 \vec{S}_1 \times \vec{v}_1 \cdot \vec{v}_2 + \right.$ 
 $2 \hat{n} \cdot \vec{v}_2 \hat{n} \cdot \vec{v}_1 \hat{n} \times \vec{S}_1 \cdot \vec{v}_1 - \frac{5}{2} \vec{v}_1 \cdot \vec{v}_1 \hat{n} \times \vec{S}_1 \cdot \vec{v}_1 + 4 \vec{v}_1 \cdot \vec{v}_1 \hat{n} \times \vec{S}_1 \cdot \vec{v}_2 + \pi^2 \left( -\frac{45}{32} (\hat{n} \cdot \vec{v}_1)^2 \hat{n} \times \vec{S}_1 \cdot \vec{v}_1 + \right.$ 
 $\left. \frac{15}{8} (\hat{n} \cdot \vec{v}_1)^2 \hat{n} \times \vec{S}_1 \cdot \vec{v}_2 + \frac{3}{4} \hat{n} \cdot \vec{v}_1 \vec{S}_1 \times \vec{v}_1 \cdot \vec{v}_2 + \frac{9}{32} \vec{v}_1 \cdot \vec{v}_1 \hat{n} \times \vec{S}_1 \cdot \vec{v}_1 - \frac{3}{8} \vec{v}_1 \cdot \vec{v}_1 \hat{n} \times \vec{S}_1 \cdot \vec{v}_2 \right) \Big) \Big\}$

{DiagSet[3, 9, 47],

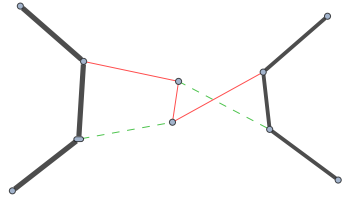

,

$$\frac{\left(\hat{n} \times \vec{a}_2 \cdot \vec{S}_1 - \frac{1}{4} \pi^2 \hat{n} \times \vec{a}_2 \cdot \vec{S}_1\right) m_1 m_2^2 G^3}{r^2} + \frac{1}{r^3} \left( \vec{a}_2 \times \vec{S}_1 \cdot \vec{v}_1 - 2 \vec{a}_2 \times \vec{S}_1 \cdot \vec{v}_2 - \hat{n} \times \vec{S}_1 \cdot \vec{v}_2 \hat{n} \cdot \vec{a}_1 - 5 \hat{n} \times \vec{S}_1 \cdot \vec{v}_1 \hat{n} \cdot \vec{a}_2 + \right. \\ \left. 5 \hat{n} \times \vec{S}_1 \cdot \vec{v}_2 \hat{n} \cdot \vec{a}_2 + 2 \hat{n} \times \vec{S}_1 \cdot \vec{v}_2 \hat{n} \cdot \vec{v}_1 + 2 \hat{n} \times \vec{S}_1 \cdot \vec{v}_1 \hat{n} \cdot \vec{v}_2 + 3 \hat{n} \times \vec{S}_1 \cdot \vec{v}_2 \hat{n} \cdot \vec{v}_2 + 3 \hat{n} \times \vec{a}_1 \cdot \vec{S}_1 \hat{n} \cdot \vec{v}_2 + \right. \\ \left. 5 \hat{n} \times \vec{a}_2 \cdot \vec{S}_1 \hat{n} \cdot \vec{v}_2 + \pi^2 \left( -\frac{1}{4} \vec{a}_2 \times \vec{S}_1 \cdot \vec{v}_1 + \frac{1}{2} \vec{a}_2 \times \vec{S}_1 \cdot \vec{v}_2 + \frac{3}{8} \hat{n} \times \vec{S}_1 \cdot \vec{v}_2 \hat{n} \cdot \vec{a}_1 + \frac{3}{4} \hat{n} \times \vec{S}_1 \cdot \vec{v}_1 \hat{n} \cdot \vec{a}_2 - \frac{3}{4} \hat{n} \times \vec{S}_1 \cdot \vec{v}_2 \hat{n} \cdot \vec{a}_2 - \right. \right. \\ \left. \left. \frac{3}{8} \hat{n} \times \vec{S}_1 \cdot \vec{v}_2 \hat{n} \cdot \vec{v}_1 - \frac{3}{8} \hat{n} \times \vec{S}_1 \cdot \vec{v}_1 \hat{n} \cdot \vec{v}_2 - \frac{3}{4} \hat{n} \times \vec{S}_1 \cdot \vec{v}_2 \hat{n} \cdot \vec{v}_2 - \frac{3}{8} \hat{n} \times \vec{a}_1 \cdot \vec{S}_1 \hat{n} \cdot \vec{v}_2 - \frac{3}{4} \hat{n} \times \vec{a}_2 \cdot \vec{S}_1 \hat{n} \cdot \vec{v}_2 \right) \right) m_1 m_2^2 G^3 + \\ \frac{1}{r^4} \left( -\frac{5}{4} \hat{n} \times \vec{S}_1 \cdot \vec{v}_2 (\hat{n} \cdot \vec{v}_1)^2 - 2 \vec{S}_1 \times \vec{v}_1 \cdot \vec{v}_2 \hat{n} \cdot \vec{v}_1 + \frac{35}{2} \hat{n} \times \vec{S}_1 \cdot \vec{v}_1 \hat{n} \cdot \vec{v}_2 \hat{n} \cdot \vec{v}_1 - \frac{23}{2} \hat{n} \times \vec{S}_1 \cdot \vec{v}_2 \hat{n} \cdot \vec{v}_2 \hat{n} \cdot \vec{v}_1 + \right. \\ \left. \frac{107}{4} \hat{n} \times \vec{S}_1 \cdot \vec{v}_1 (\hat{n} \cdot \vec{v}_2)^2 + \frac{13}{2} \hat{n} \times \vec{S}_1 \cdot \vec{v}_2 (\hat{n} \cdot \vec{v}_2)^2 - 10 \vec{S}_1 \times \vec{v}_1 \cdot \vec{v}_2 \hat{n} \cdot \vec{v}_2 + \frac{1}{4} \hat{n} \times \vec{S}_1 \cdot \vec{v}_2 \vec{v}_1 \cdot \vec{v}_1 - \right. \\ \left. \frac{11}{2} \hat{n} \times \vec{S}_1 \cdot \vec{v}_1 \vec{v}_1 \cdot \vec{v}_2 + \frac{9}{2} \hat{n} \times \vec{S}_1 \cdot \vec{v}_2 \vec{v}_1 \cdot \vec{v}_2 - \frac{19}{4} \hat{n} \times \vec{S}_1 \cdot \vec{v}_1 \vec{v}_2 \cdot \vec{v}_2 - \frac{1}{2} \hat{n} \times \vec{S}_1 \cdot \vec{v}_2 \vec{v}_2 \cdot \vec{v}_2 + \right. \\ \left. \pi^2 \left( -\frac{15}{64} \hat{n} \times \vec{S}_1 \cdot \vec{v}_2 (\hat{n} \cdot \vec{v}_1)^2 + \frac{3}{8} \vec{S}_1 \times \vec{v}_1 \cdot \vec{v}_2 \hat{n} \cdot \vec{v}_1 - \frac{75}{32} \hat{n} \times \vec{S}_1 \cdot \vec{v}_1 \hat{n} \cdot \vec{v}_2 \hat{n} \cdot \vec{v}_1 + \frac{45}{32} \hat{n} \times \vec{S}_1 \cdot \vec{v}_2 \hat{n} \cdot \vec{v}_2 \hat{n} \cdot \vec{v}_1 - \right. \right. \\ \left. \left. \frac{255}{64} \hat{n} \times \vec{S}_1 \cdot \vec{v}_1 (\hat{n} \cdot \vec{v}_2)^2 - \frac{75}{32} \hat{n} \times \vec{S}_1 \cdot \vec{v}_2 (\hat{n} \cdot \vec{v}_2)^2 + \frac{15}{8} \vec{S}_1 \times \vec{v}_1 \cdot \vec{v}_2 \hat{n} \cdot \vec{v}_2 + \frac{3}{64} \hat{n} \times \vec{S}_1 \cdot \vec{v}_2 \vec{v}_1 \cdot \vec{v}_1 + \right. \right. \\ \left. \left. \frac{15}{32} \hat{n} \times \vec{S}_1 \cdot \vec{v}_1 \vec{v}_1 \cdot \vec{v}_2 - \frac{9}{32} \hat{n} \times \vec{S}_1 \cdot \vec{v}_2 \vec{v}_1 \cdot \vec{v}_2 + \frac{51}{64} \hat{n} \times \vec{S}_1 \cdot \vec{v}_1 \vec{v}_2 \cdot \vec{v}_2 + \frac{15}{32} \hat{n} \times \vec{S}_1 \cdot \vec{v}_2 \vec{v}_2 \cdot \vec{v}_2 \right) \right) m_1 m_2^2 G^3 \Big\}$$

{DiagSet[3, 9, 48],

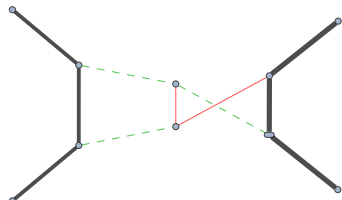

,

$$\frac{1}{r^3} G^3 m_1 m_2^2 \left( -4 \hat{n} \cdot \vec{a}_2 \hat{n} \times \vec{S}_1 \cdot \vec{v}_2 - 20 \hat{n} \cdot \vec{v}_2 \hat{n} \times \vec{S}_1 \cdot \vec{a}_2 + \pi^2 \left( \frac{3}{2} \hat{n} \cdot \vec{a}_2 \hat{n} \times \vec{S}_1 \cdot \vec{v}_2 - \frac{1}{2} \vec{S}_1 \times \vec{v}_2 \cdot \vec{a}_2 + \frac{3}{2} \hat{n} \cdot \vec{v}_2 \hat{n} \times \vec{S}_1 \cdot \vec{v}_2 \right) - \right. \\ \left. 24 \hat{n} \cdot \vec{v}_2 \hat{n} \times \vec{S}_1 \cdot \vec{v}_2 \right) + \frac{1}{r^4} G^3 m_1 m_2^2 \left( -45 (\hat{n} \cdot \vec{v}_2)^2 \hat{n} \times \vec{S}_1 \cdot \vec{v}_1 - 89 (\hat{n} \cdot \vec{v}_2)^2 \hat{n} \times \vec{S}_1 \cdot \vec{v}_2 + \right. \\ \left. 44 \hat{n} \cdot \vec{v}_2 \vec{S}_1 \times \vec{v}_1 \cdot \vec{v}_2 + 94 \hat{n} \cdot \vec{v}_1 \hat{n} \cdot \vec{v}_2 \hat{n} \times \vec{S}_1 \cdot \vec{v}_2 - 14 \vec{v}_1 \cdot \vec{v}_2 \hat{n} \times \vec{S}_1 \cdot \vec{v}_2 + 5 \vec{v}_2 \cdot \vec{v}_2 \hat{n} \times \vec{S}_1 \cdot \vec{v}_1 + \right. \\ \left. 9 \vec{v}_2 \cdot \vec{v}_2 \hat{n} \times \vec{S}_1 \cdot \vec{v}_2 + \pi^2 \left( \frac{105}{16} (\hat{n} \cdot \vec{v}_2)^2 \hat{n} \times \vec{S}_1 \cdot \vec{v}_1 + \frac{105}{16} (\hat{n} \cdot \vec{v}_2)^2 \hat{n} \times \vec{S}_1 \cdot \vec{v}_2 - \frac{15}{4} \hat{n} \cdot \vec{v}_2 \vec{S}_1 \times \vec{v}_1 \cdot \vec{v}_2 - \right. \right. \\ \left. \left. \frac{45}{8} \hat{n} \cdot \vec{v}_1 \hat{n} \cdot \vec{v}_2 \hat{n} \times \vec{S}_1 \cdot \vec{v}_2 + \frac{9}{8} \vec{v}_1 \cdot \vec{v}_2 \hat{n} \times \vec{S}_1 \cdot \vec{v}_2 - \frac{21}{16} \vec{v}_2 \cdot \vec{v}_2 \hat{n} \times \vec{S}_1 \cdot \vec{v}_1 - \frac{21}{16} \vec{v}_2 \cdot \vec{v}_2 \hat{n} \times \vec{S}_1 \cdot \vec{v}_2 \right) \right) \Big\}$$

{DiagSet[3, 9, 49],

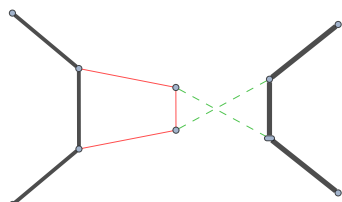

,

$$\begin{aligned}
& \frac{\left( \frac{1}{4} \pi^2 \hat{n} \times \vec{S}_1 \cdot \vec{a}_1 - \hat{n} \times \vec{S}_1 \cdot \vec{a}_1 \right) m_1 m_2^2 G^3}{r^2} + \frac{1}{r^3} \left( - \left( \vec{S}_1 \times \vec{v}_1 \cdot \vec{v}_2 \right) + \vec{S}_1 \times \vec{a}_1 \cdot \vec{v}_2 + \vec{S}_1 \times \vec{v}_1 \cdot \vec{a}_1 - \vec{S}_1 \times \vec{v}_1 \cdot \vec{a}_2 - \right. \\
& \hat{n} \times \vec{S}_1 \cdot \vec{v}_1 \hat{n} \cdot \vec{a}_1 + 5 \hat{n} \times \vec{S}_1 \cdot \vec{v}_2 \hat{n} \cdot \vec{a}_1 + 2 \hat{n} \times \vec{S}_1 \cdot \vec{v}_1 \hat{n} \cdot \vec{a}_2 - 4 \hat{n} \times \vec{S}_1 \cdot \vec{v}_2 \hat{n} \cdot \vec{v}_1 + 4 \hat{n} \times \vec{S}_1 \cdot \vec{a}_1 \hat{n} \cdot \vec{v}_1 + \\
& \hat{n} \times \vec{S}_1 \cdot \vec{a}_2 \hat{n} \cdot \vec{v}_1 + \pi^2 \left( \frac{1}{4} \vec{S}_1 \times \vec{v}_1 \cdot \vec{v}_2 - \frac{1}{4} \vec{S}_1 \times \vec{a}_1 \cdot \vec{v}_2 - \frac{1}{4} \vec{S}_1 \times \vec{v}_1 \cdot \vec{a}_1 + \frac{1}{4} \vec{S}_1 \times \vec{v}_1 \cdot \vec{a}_2 - \frac{3}{4} \hat{n} \times \vec{S}_1 \cdot \vec{v}_2 \hat{n} \cdot \vec{a}_1 - \right. \\
& \left. \frac{3}{4} \hat{n} \times \vec{S}_1 \cdot \vec{v}_1 \hat{n} \cdot \vec{a}_2 + \frac{3}{4} \hat{n} \times \vec{S}_1 \cdot \vec{v}_2 \hat{n} \cdot \vec{v}_1 - \frac{3}{4} \hat{n} \times \vec{S}_1 \cdot \vec{a}_1 \hat{n} \cdot \vec{v}_1 \right) - \hat{n} \times \vec{S}_1 \cdot \vec{v}_1 \hat{n} \cdot \vec{v}_2 \left. \right) m_1 m_2^2 G^3 + \frac{1}{r^4} \\
& \left( - \frac{17}{4} \hat{n} \times \vec{S}_1 \cdot \vec{v}_1 (\hat{n} \cdot \vec{v}_1)^2 + \frac{65}{4} \hat{n} \times \vec{S}_1 \cdot \vec{v}_2 (\hat{n} \cdot \vec{v}_1)^2 + 7 \vec{S}_1 \times \vec{v}_1 \cdot \vec{v}_2 \hat{n} \cdot \vec{v}_1 - \frac{25}{2} \hat{n} \times \vec{S}_1 \cdot \vec{v}_1 \hat{n} \cdot \vec{v}_2 \hat{n} \cdot \vec{v}_1 + \right. \\
& 10 \hat{n} \times \vec{S}_1 \cdot \vec{v}_2 \hat{n} \cdot \vec{v}_2 \hat{n} \cdot \vec{v}_1 - \frac{5}{2} \hat{n} \times \vec{S}_1 \cdot \vec{v}_1 (\hat{n} \cdot \vec{v}_2)^2 + \vec{S}_1 \times \vec{v}_1 \cdot \vec{v}_2 \hat{n} \cdot \vec{v}_2 + \frac{5}{4} \hat{n} \times \vec{S}_1 \cdot \vec{v}_1 \vec{v}_1 \cdot \vec{v}_1 - \\
& \frac{13}{4} \hat{n} \times \vec{S}_1 \cdot \vec{v}_2 \vec{v}_1 \cdot \vec{v}_1 + \frac{9}{2} \hat{n} \times \vec{S}_1 \cdot \vec{v}_1 \vec{v}_1 \cdot \vec{v}_2 - 6 \hat{n} \times \vec{S}_1 \cdot \vec{v}_2 \vec{v}_1 \cdot \vec{v}_2 + \frac{1}{2} \hat{n} \times \vec{S}_1 \cdot \vec{v}_1 \vec{v}_2 \cdot \vec{v}_2 + \\
& \pi^2 \left( \frac{45}{64} \hat{n} \times \vec{S}_1 \cdot \vec{v}_1 (\hat{n} \cdot \vec{v}_1)^2 - \frac{165}{64} \hat{n} \times \vec{S}_1 \cdot \vec{v}_2 (\hat{n} \cdot \vec{v}_1)^2 - \frac{3}{2} \vec{S}_1 \times \vec{v}_1 \cdot \vec{v}_2 \hat{n} \cdot \vec{v}_1 + \frac{75}{32} \hat{n} \times \vec{S}_1 \cdot \vec{v}_1 \hat{n} \cdot \vec{v}_2 \hat{n} \cdot \vec{v}_1 - \right. \\
& \frac{15}{16} \hat{n} \times \vec{S}_1 \cdot \vec{v}_2 \hat{n} \cdot \vec{v}_2 \hat{n} \cdot \vec{v}_1 - \frac{15}{32} \hat{n} \times \vec{S}_1 \cdot \vec{v}_1 (\hat{n} \cdot \vec{v}_2)^2 - \frac{9}{64} \hat{n} \times \vec{S}_1 \cdot \vec{v}_1 \vec{v}_1 \cdot \vec{v}_1 + \frac{33}{64} \hat{n} \times \vec{S}_1 \cdot \vec{v}_2 \vec{v}_1 \cdot \vec{v}_1 - \\
& \left. \frac{15}{32} \hat{n} \times \vec{S}_1 \cdot \vec{v}_1 \vec{v}_1 \cdot \vec{v}_2 + \frac{3}{16} \hat{n} \times \vec{S}_1 \cdot \vec{v}_2 \vec{v}_1 \cdot \vec{v}_2 + \frac{3}{32} \hat{n} \times \vec{S}_1 \cdot \vec{v}_1 \vec{v}_2 \cdot \vec{v}_2 \right) \left. \right) m_1 m_2^2 G^3 \}
\end{aligned}$$

$\{ \text{DiagSet}[3, 9, 50],$ 
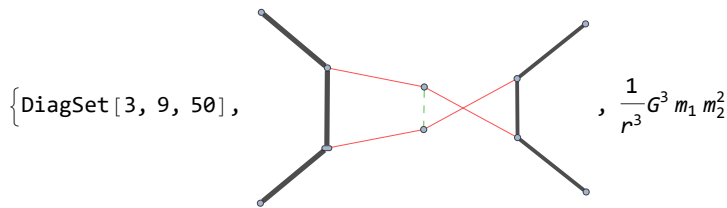
 $, \frac{1}{r^3} G^3 m_1 m_2^2$

$$\begin{aligned}
& \left( -2 \hat{n} \cdot \vec{v}_1 \hat{n} \times \vec{a}_1 \cdot \vec{S}_1 - \hat{n} \cdot \vec{v}_2 \hat{n} \times \vec{a}_1 \cdot \vec{S}_1 - 2 \vec{a}_1 \times \vec{S}_1 \cdot \vec{v}_1 - \vec{a}_1 \times \vec{S}_1 \cdot \vec{v}_2 + 2 \hat{n} \cdot \vec{v}_1 \hat{n} \times \vec{S}_1 \cdot \vec{v}_1 + \hat{n} \cdot \vec{v}_2 \hat{n} \times \vec{S}_1 \cdot \vec{v}_1 + \vec{S}_1 \times \vec{v}_1 \cdot \vec{v}_2 \right) + \\
& \frac{1}{r^4} G^3 m_1 m_2^2 \left( -5 (\hat{n} \cdot \vec{v}_1)^2 \hat{n} \times \vec{S}_1 \cdot \vec{v}_1 + \hat{n} \cdot \vec{v}_1 \vec{S}_1 \times \vec{v}_1 \cdot \vec{v}_2 - 5 \hat{n} \cdot \vec{v}_2 \hat{n} \cdot \vec{v}_1 \hat{n} \times \vec{S}_1 \cdot \vec{v}_1 - 5 (\hat{n} \cdot \vec{v}_2)^2 \hat{n} \times \vec{S}_1 \cdot \vec{v}_1 + \right. \\
& \left. 2 \hat{n} \cdot \vec{v}_2 \vec{S}_1 \times \vec{v}_1 \cdot \vec{v}_2 - 3 \vec{v}_1 \cdot \vec{v}_1 \hat{n} \times \vec{S}_1 \cdot \vec{v}_1 - 3 \vec{v}_1 \cdot \vec{v}_2 \hat{n} \times \vec{S}_1 \cdot \vec{v}_1 - 3 \vec{v}_2 \cdot \vec{v}_2 \hat{n} \times \vec{S}_1 \cdot \vec{v}_1 \right) \}
\end{aligned}$$

$\{ \text{DiagSet}[3, 9, 51],$ 
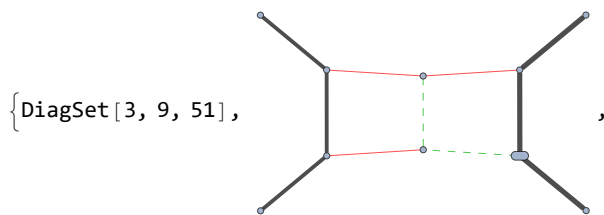
 $,$

$$\begin{aligned}
& \frac{1}{r^3} G^3 m_1 m_2^2 \left( -2 \hat{n} \cdot \vec{v}_1 \hat{n} \times \vec{S}_1 \cdot \vec{a}_1 + 2 \hat{n} \cdot \vec{v}_2 \hat{n} \times \vec{S}_1 \cdot \vec{a}_1 + \pi^2 \left( -\frac{3}{2} \hat{n} \cdot \vec{v}_1 \hat{n} \times \vec{S}_1 \cdot \vec{a}_1 - \frac{3}{2} \hat{n} \cdot \vec{v}_2 \hat{n} \times \vec{S}_1 \cdot \vec{a}_1 + \right. \right. \\
& \left. \frac{1}{2} \vec{S}_1 \times \vec{a}_1 \cdot \vec{v}_2 - \frac{1}{2} \vec{S}_1 \times \vec{v}_1 \cdot \vec{a}_1 - \frac{3}{2} \hat{n} \cdot \vec{v}_1 \hat{n} \times \vec{S}_1 \cdot \vec{v}_1 - \frac{3}{2} \hat{n} \cdot \vec{v}_2 \hat{n} \times \vec{S}_1 \cdot \vec{v}_1 + \frac{1}{2} \vec{S}_1 \times \vec{v}_1 \cdot \vec{v}_2 \right) + \\
& \left. 2 \vec{S}_1 \times \vec{a}_1 \cdot \vec{v}_2 + 2 \vec{S}_1 \times \vec{v}_1 \cdot \vec{a}_1 - 2 \hat{n} \cdot \vec{v}_1 \hat{n} \times \vec{S}_1 \cdot \vec{v}_1 + 2 \hat{n} \cdot \vec{v}_2 \hat{n} \times \vec{S}_1 \cdot \vec{v}_1 + 2 \vec{S}_1 \times \vec{v}_1 \cdot \vec{v}_2 \right) + \frac{1}{r^4} \\
& G^3 m_1 m_2^2 \left( \hat{n} \cdot \vec{v}_1 \vec{S}_1 \times \vec{v}_1 \cdot \vec{v}_2 - 10 \hat{n} \cdot \vec{v}_2 \hat{n} \cdot \vec{v}_1 \hat{n} \times \vec{S}_1 \cdot \vec{v}_1 + 6 \vec{v}_1 \cdot \vec{v}_1 \hat{n} \times \vec{S}_1 \cdot \vec{v}_1 - 3 \vec{v}_1 \cdot \vec{v}_1 \hat{n} \times \vec{S}_1 \cdot \vec{v}_2 - \right. \\
& \left. \vec{v}_1 \cdot \vec{v}_2 \hat{n} \times \vec{S}_1 \cdot \vec{v}_1 + \pi^2 \left( \frac{15}{4} (\hat{n} \cdot \vec{v}_1)^2 \hat{n} \times \vec{S}_1 \cdot \vec{v}_1 - \frac{3}{4} \hat{n} \cdot \vec{v}_1 \vec{S}_1 \times \vec{v}_1 \cdot \vec{v}_2 + \frac{15}{4} \hat{n} \cdot \vec{v}_2 \hat{n} \cdot \vec{v}_1 \hat{n} \times \vec{S}_1 \cdot \vec{v}_1 - \right. \right.
\end{aligned}$$

$$\frac{3}{4} \vec{v}_1 \cdot \vec{v}_1 \hat{n} \times \vec{S}_1 \cdot \vec{v}_1 - \frac{3}{4} \vec{v}_1 \cdot \vec{v}_2 \hat{n} \times \vec{S}_1 \cdot \vec{v}_1 \Big) + 6 \vec{v}_2 \cdot \vec{v}_2 \hat{n} \times \vec{S}_1 \cdot \vec{v}_1 - 6 \vec{v}_2 \cdot \vec{v}_2 \hat{n} \times \vec{S}_1 \cdot \vec{v}_2 \Big) \Big\}$$

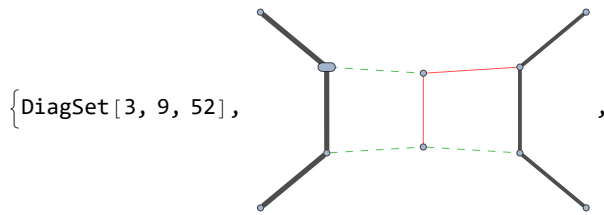

$$\frac{1}{r^3} G^3 m_1 m_2^2 \left( -8 \hat{n} \cdot \vec{a}_1 \hat{n} \times \vec{S}_1 \cdot \vec{v}_2 + 8 \hat{n} \cdot \vec{a}_2 \hat{n} \times \vec{S}_1 \cdot \vec{v}_1 - 8 \hat{n} \cdot \vec{v}_1 \hat{n} \times \vec{S}_1 \cdot \vec{a}_2 + 8 \hat{n} \cdot \vec{v}_2 \hat{n} \times \vec{S}_1 \cdot \vec{a}_1 \right) +$$

$$\frac{1}{r^4} G^3 m_1 m_2^2 \left( 20 (\hat{n} \cdot \vec{v}_1)^2 \hat{n} \times \vec{S}_1 \cdot \vec{v}_2 - 20 \hat{n} \cdot \vec{v}_2 \hat{n} \cdot \vec{v}_1 \hat{n} \times \vec{S}_1 \cdot \vec{v}_1 + \right.$$

$$\left. 8 \hat{n} \cdot \vec{v}_2 \vec{S}_1 \times \vec{v}_1 \cdot \vec{v}_2 - 8 \vec{v}_1 \cdot \vec{v}_1 \hat{n} \times \vec{S}_1 \cdot \vec{v}_2 + 4 \vec{v}_1 \cdot \vec{v}_2 \hat{n} \times \vec{S}_1 \cdot \vec{v}_1 - 8 \vec{v}_2 \cdot \vec{v}_2 \hat{n} \times \vec{S}_1 \cdot \vec{v}_1 \right) \Big\}$$

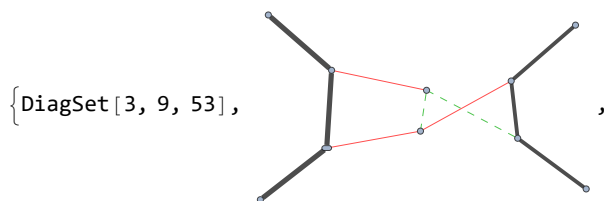

$$\frac{1}{r^3} G^3 m_1 m_2^2 \left( -4 \hat{n} \cdot \vec{v}_2 \hat{n} \times \vec{a}_1 \cdot \vec{S}_1 + \pi^2 \left( 3 \hat{n} \cdot \vec{v}_2 \hat{n} \times \vec{a}_1 \cdot \vec{S}_1 - \vec{a}_1 \times \vec{S}_1 \cdot \vec{v}_2 - 3 \hat{n} \cdot \vec{v}_2 \hat{n} \times \vec{S}_1 \cdot \vec{v}_1 + \vec{S}_1 \times \vec{v}_1 \cdot \vec{v}_2 \right) - \right.$$

$$\left. 4 \vec{a}_1 \times \vec{S}_1 \cdot \vec{v}_2 + 4 \hat{n} \cdot \vec{v}_2 \hat{n} \times \vec{S}_1 \cdot \vec{v}_1 + 4 \vec{S}_1 \times \vec{v}_1 \cdot \vec{v}_2 \right) + \frac{1}{r^4}$$

$$G^3 m_1 m_2^2 \left( -4 \hat{n} \cdot \vec{v}_1 \vec{S}_1 \times \vec{v}_1 \cdot \vec{v}_2 - 20 \hat{n} \cdot \vec{v}_2 \hat{n} \cdot \vec{v}_1 \hat{n} \times \vec{S}_1 \cdot \vec{v}_1 - 8 \hat{n} \cdot \vec{v}_2 \vec{S}_1 \times \vec{v}_1 \cdot \vec{v}_2 - 4 \vec{v}_1 \cdot \vec{v}_2 \hat{n} \times \vec{S}_1 \cdot \vec{v}_1 + \right.$$

$$\left. 8 \vec{v}_2 \cdot \vec{v}_2 \hat{n} \times \vec{S}_1 \cdot \vec{v}_1 + \pi^2 \left( 15 (\hat{n} \cdot \vec{v}_2)^2 \hat{n} \times \vec{S}_1 \cdot \vec{v}_1 - 6 \hat{n} \cdot \vec{v}_2 \vec{S}_1 \times \vec{v}_1 \cdot \vec{v}_2 + \right. \right.$$

$$\left. \left. 15 \hat{n} \cdot \vec{v}_1 \hat{n} \cdot \vec{v}_2 \hat{n} \times \vec{S}_1 \cdot \vec{v}_1 - 3 \hat{n} \cdot \vec{v}_1 \vec{S}_1 \times \vec{v}_1 \cdot \vec{v}_2 - 3 \vec{v}_1 \cdot \vec{v}_2 \hat{n} \times \vec{S}_1 \cdot \vec{v}_1 - 3 \vec{v}_2 \cdot \vec{v}_2 \hat{n} \times \vec{S}_1 \cdot \vec{v}_1 \right) \right) \Big\}$$

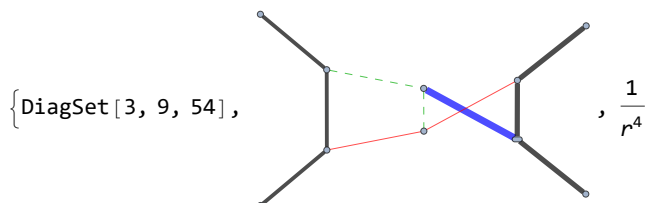

$$G^3 m_1 m_2^2 \left( -\frac{19}{2} (\hat{n} \cdot \vec{v}_1)^2 \hat{n} \times \vec{S}_1 \cdot \vec{v}_2 - 6 \hat{n} \cdot \vec{v}_1 \vec{S}_1 \times \vec{v}_1 \cdot \vec{v}_2 + \hat{n} \cdot \vec{v}_2 \hat{n} \cdot \vec{v}_1 \hat{n} \times \vec{S}_1 \cdot \vec{v}_1 - 14 \hat{n} \cdot \vec{v}_2 \hat{n} \cdot \vec{v}_1 \hat{n} \times \vec{S}_1 \cdot \vec{v}_2 + \frac{1}{2} (\hat{n} \cdot \vec{v}_2)^2 \right.$$

$$\left. \hat{n} \times \vec{S}_1 \cdot \vec{v}_1 - 5 \hat{n} \cdot \vec{v}_2 \vec{S}_1 \times \vec{v}_1 \cdot \vec{v}_2 + \frac{3}{2} \vec{v}_1 \cdot \vec{v}_1 \hat{n} \times \vec{S}_1 \cdot \vec{v}_2 + \vec{v}_1 \cdot \vec{v}_2 \hat{n} \times \vec{S}_1 \cdot \vec{v}_1 + 6 \vec{v}_1 \cdot \vec{v}_2 \hat{n} \times \vec{S}_1 \cdot \vec{v}_2 - \frac{5}{2} \vec{v}_2 \cdot \vec{v}_2 \hat{n} \times \vec{S}_1 \cdot \vec{v}_1 + \right.$$

$$\pi^2 \left( \frac{15}{32} (\hat{n} \cdot \vec{v}_1)^2 \hat{n} \times \vec{S}_1 \cdot \vec{v}_2 + \frac{15}{16} \hat{n} \cdot \vec{v}_2 \hat{n} \cdot \vec{v}_1 \hat{n} \times \vec{S}_1 \cdot \vec{v}_1 + \frac{15}{16} \hat{n} \cdot \vec{v}_2 \hat{n} \cdot \vec{v}_1 \hat{n} \times \vec{S}_1 \cdot \vec{v}_2 + \frac{15}{32} (\hat{n} \cdot \vec{v}_2)^2 \hat{n} \times \vec{S}_1 \cdot \vec{v}_1 - \right.$$

$$\left. \frac{3}{32} \vec{v}_1 \cdot \vec{v}_1 \hat{n} \times \vec{S}_1 \cdot \vec{v}_2 - \frac{3}{16} \vec{v}_1 \cdot \vec{v}_2 \hat{n} \times \vec{S}_1 \cdot \vec{v}_1 - \frac{3}{16} \vec{v}_1 \cdot \vec{v}_2 \hat{n} \times \vec{S}_1 \cdot \vec{v}_2 - \frac{3}{32} \vec{v}_2 \cdot \vec{v}_2 \hat{n} \times \vec{S}_1 \cdot \vec{v}_1 \right) \Big\}$$

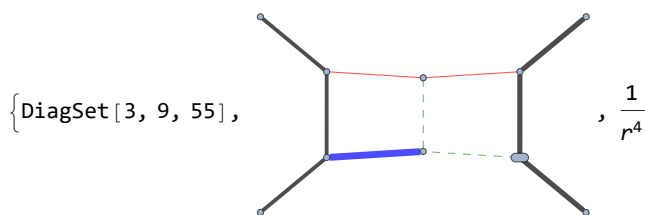

$$G^3 m_1 m_2^2 \left( -\frac{27}{4} (\hat{n} \cdot \vec{v}_2)^2 \hat{n} \times \vec{S}_1 \cdot \vec{v}_1 + \frac{43}{4} (\hat{n} \cdot \vec{v}_2)^2 \hat{n} \times \vec{S}_1 \cdot \vec{v}_2 + 4 \hat{n} \cdot \vec{v}_2 \vec{S}_1 \times \vec{v}_1 \cdot \vec{v}_2 + \right. \\ \left. \frac{13}{2} \hat{n} \cdot \vec{v}_1 \hat{n} \cdot \vec{v}_2 \hat{n} \times \vec{S}_1 \cdot \vec{v}_2 + \frac{3}{2} \vec{v}_1 \cdot \vec{v}_2 \hat{n} \times \vec{S}_1 \cdot \vec{v}_2 - \frac{1}{4} \vec{v}_2 \cdot \vec{v}_2 \hat{n} \times \vec{S}_1 \cdot \vec{v}_1 - \frac{7}{4} \vec{v}_2 \cdot \vec{v}_2 \hat{n} \times \vec{S}_1 \cdot \vec{v}_2 + \right. \\ \left. \pi^2 \left( \frac{75}{64} (\hat{n} \cdot \vec{v}_2)^2 \hat{n} \times \vec{S}_1 \cdot \vec{v}_1 - \frac{75}{64} (\hat{n} \cdot \vec{v}_2)^2 \hat{n} \times \vec{S}_1 \cdot \vec{v}_2 - \frac{3}{8} \hat{n} \cdot \vec{v}_2 \vec{S}_1 \times \vec{v}_1 \cdot \vec{v}_2 + \right. \right. \\ \left. \left. \frac{15}{32} \hat{n} \cdot \vec{v}_1 \hat{n} \cdot \vec{v}_2 \hat{n} \times \vec{S}_1 \cdot \vec{v}_2 - \frac{3}{32} \vec{v}_1 \cdot \vec{v}_2 \hat{n} \times \vec{S}_1 \cdot \vec{v}_2 - \frac{15}{64} \vec{v}_2 \cdot \vec{v}_2 \hat{n} \times \vec{S}_1 \cdot \vec{v}_1 + \frac{15}{64} \vec{v}_2 \cdot \vec{v}_2 \hat{n} \times \vec{S}_1 \cdot \vec{v}_2 \right) \right) \Bigg\}$$

{DiagSet[3, 9, 56],

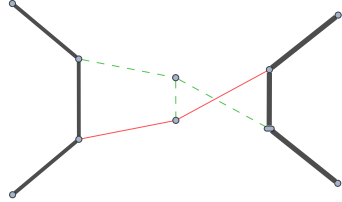

,

$$\frac{1}{r^3} \left( 3 \vec{S}_1 \times \vec{v}_1 \cdot \vec{v}_2 + 5 \vec{S}_1 \times \vec{a}_1 \cdot \vec{v}_2 - \vec{S}_1 \times \vec{v}_1 \cdot \vec{a}_2 - 8 \vec{S}_1 \times \vec{v}_2 \cdot \vec{a}_2 + 7 \hat{n} \times \vec{S}_1 \cdot \vec{v}_2 \hat{n} \cdot \vec{a}_1 - \hat{n} \times \vec{S}_1 \cdot \vec{v}_1 \hat{n} \cdot \vec{a}_2 + 8 \hat{n} \times \vec{S}_1 \cdot \vec{v}_2 \hat{n} \cdot \vec{a}_2 + \right. \\ \left. 2 \hat{n} \times \vec{S}_1 \cdot \vec{a}_2 \hat{n} \cdot \vec{v}_1 - 3 \hat{n} \times \vec{S}_1 \cdot \vec{v}_1 \hat{n} \cdot \vec{v}_2 + 2 \hat{n} \times \vec{S}_1 \cdot \vec{v}_2 \hat{n} \cdot \vec{v}_2 - 6 \hat{n} \times \vec{S}_1 \cdot \vec{a}_1 \hat{n} \cdot \vec{v}_2 - 16 \hat{n} \times \vec{S}_1 \cdot \vec{a}_2 \hat{n} \cdot \vec{v}_2 + \right. \\ \left. \pi^2 \left( -\frac{1}{4} \vec{S}_1 \times \vec{v}_1 \cdot \vec{v}_2 - \frac{1}{4} \vec{S}_1 \times \vec{a}_1 \cdot \vec{v}_2 - \frac{1}{8} \vec{S}_1 \times \vec{v}_1 \cdot \vec{a}_2 + \frac{1}{2} \vec{S}_1 \times \vec{v}_2 \cdot \vec{a}_2 - \frac{3}{8} \hat{n} \times \vec{S}_1 \cdot \vec{v}_2 \hat{n} \cdot \vec{a}_1 - \frac{3}{8} \hat{n} \times \vec{S}_1 \cdot \vec{v}_2 \hat{n} \cdot \vec{v}_1 - \right. \right. \\ \left. \left. \frac{3}{8} \hat{n} \times \vec{S}_1 \cdot \vec{a}_2 \hat{n} \cdot \vec{v}_1 + \frac{3}{8} \hat{n} \times \vec{S}_1 \cdot \vec{v}_1 \hat{n} \cdot \vec{v}_2 - \frac{3}{4} \hat{n} \times \vec{S}_1 \cdot \vec{v}_2 \hat{n} \cdot \vec{v}_2 + \frac{3}{8} \hat{n} \times \vec{S}_1 \cdot \vec{a}_1 \hat{n} \cdot \vec{v}_2 + \frac{3}{2} \hat{n} \times \vec{S}_1 \cdot \vec{a}_2 \hat{n} \cdot \vec{v}_2 \right) \right) m_1 m_2^2 G^3 + \\ \frac{1}{r^4} \left( -\frac{41}{2} \hat{n} \times \vec{S}_1 \cdot \vec{v}_2 (\hat{n} \cdot \vec{v}_1)^2 - 17 \vec{S}_1 \times \vec{v}_1 \cdot \vec{v}_2 \hat{n} \cdot \vec{v}_1 + 34 \hat{n} \times \vec{S}_1 \cdot \vec{v}_1 \hat{n} \cdot \vec{v}_2 \hat{n} \cdot \vec{v}_1 + 12 \hat{n} \times \vec{S}_1 \cdot \vec{v}_2 \hat{n} \cdot \vec{v}_2 \hat{n} \cdot \vec{v}_1 - \right. \\ \left. \frac{3}{2} \hat{n} \times \vec{S}_1 \cdot \vec{v}_1 (\hat{n} \cdot \vec{v}_2)^2 + \frac{5}{2} \hat{n} \times \vec{S}_1 \cdot \vec{v}_2 (\hat{n} \cdot \vec{v}_2)^2 + 5 \vec{S}_1 \times \vec{v}_1 \cdot \vec{v}_2 \hat{n} \cdot \vec{v}_2 + \frac{13}{2} \hat{n} \times \vec{S}_1 \cdot \vec{v}_2 \vec{v}_1 \cdot \vec{v}_1 - \right. \\ \left. 6 \hat{n} \times \vec{S}_1 \cdot \vec{v}_1 \vec{v}_1 \cdot \vec{v}_2 + 2 \hat{n} \times \vec{S}_1 \cdot \vec{v}_2 \vec{v}_1 \cdot \vec{v}_2 - \frac{5}{2} \hat{n} \times \vec{S}_1 \cdot \vec{v}_1 \vec{v}_2 \cdot \vec{v}_2 - \frac{1}{2} \hat{n} \times \vec{S}_1 \cdot \vec{v}_2 \vec{v}_2 \cdot \vec{v}_2 + \right. \\ \left. \pi^2 \left( \frac{45}{32} \hat{n} \times \vec{S}_1 \cdot \vec{v}_2 (\hat{n} \cdot \vec{v}_1)^2 + \frac{9}{8} \vec{S}_1 \times \vec{v}_1 \cdot \vec{v}_2 \hat{n} \cdot \vec{v}_1 - \frac{45}{16} \hat{n} \times \vec{S}_1 \cdot \vec{v}_1 \hat{n} \cdot \vec{v}_2 \hat{n} \cdot \vec{v}_1 - \frac{15}{16} \hat{n} \times \vec{S}_1 \cdot \vec{v}_2 \hat{n} \cdot \vec{v}_2 \hat{n} \cdot \vec{v}_1 + \right. \right. \\ \left. \left. \frac{15}{32} \hat{n} \times \vec{S}_1 \cdot \vec{v}_1 (\hat{n} \cdot \vec{v}_2)^2 + \frac{45}{32} \hat{n} \times \vec{S}_1 \cdot \vec{v}_2 (\hat{n} \cdot \vec{v}_2)^2 - \frac{3}{8} \vec{S}_1 \times \vec{v}_1 \cdot \vec{v}_2 \hat{n} \cdot \vec{v}_2 - \frac{9}{32} \hat{n} \times \vec{S}_1 \cdot \vec{v}_2 \vec{v}_1 \cdot \vec{v}_1 + \right. \right. \\ \left. \left. \frac{9}{16} \hat{n} \times \vec{S}_1 \cdot \vec{v}_1 \vec{v}_1 \cdot \vec{v}_2 + \frac{3}{16} \hat{n} \times \vec{S}_1 \cdot \vec{v}_2 \vec{v}_1 \cdot \vec{v}_2 - \frac{3}{32} \hat{n} \times \vec{S}_1 \cdot \vec{v}_1 \vec{v}_2 \cdot \vec{v}_2 - \frac{9}{32} \hat{n} \times \vec{S}_1 \cdot \vec{v}_2 \vec{v}_2 \cdot \vec{v}_2 \right) \right) m_1 m_2^2 G^3 \Bigg\}$$

{DiagSet[3, 9, 57],

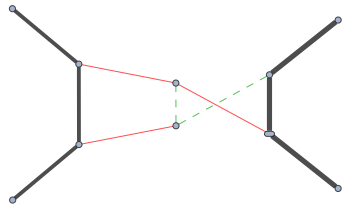

,  $\frac{1}{r^3} G^3 m_1 m_2^2$

$$\left( -4 \hat{n} \cdot \vec{v}_1 \hat{n} \times \vec{S}_1 \cdot \vec{a}_1 + \pi^2 \left( -3 \hat{n} \cdot \vec{v}_1 \hat{n} \times \vec{S}_1 \cdot \vec{a}_1 - (\vec{S}_1 \times \vec{v}_1 \cdot \vec{a}_1) - 3 \hat{n} \cdot \vec{v}_1 \hat{n} \times \vec{S}_1 \cdot \vec{v}_1 \right) + 4 \vec{S}_1 \times \vec{v}_1 \cdot \vec{a}_1 - 4 \hat{n} \cdot \vec{v}_1 \hat{n} \times \vec{S}_1 \cdot \vec{v}_1 \right) + \\ \frac{1}{r^4} G^3 m_1 m_2^2 \left( 20 (\hat{n} \cdot \vec{v}_1)^2 \hat{n} \times \vec{S}_1 \cdot \vec{v}_1 + 4 \vec{v}_1 \cdot \vec{v}_1 \hat{n} \times \vec{S}_1 \cdot \vec{v}_1 - 8 \vec{v}_1 \cdot \vec{v}_2 \hat{n} \times \vec{S}_1 \cdot \vec{v}_1 + \pi^2 \left( \frac{15}{2} (\hat{n} \cdot \vec{v}_1)^2 \hat{n} \times \vec{S}_1 \cdot \vec{v}_1 - \right. \right. \\ \left. \left. \frac{3}{2} \hat{n} \cdot \vec{v}_1 \vec{S}_1 \times \vec{v}_1 \cdot \vec{v}_2 + \frac{15}{2} \hat{n} \cdot \vec{v}_2 \hat{n} \cdot \vec{v}_1 \hat{n} \times \vec{S}_1 \cdot \vec{v}_1 - \frac{3}{2} \vec{v}_1 \cdot \vec{v}_1 \hat{n} \times \vec{S}_1 \cdot \vec{v}_1 - \frac{3}{2} \vec{v}_1 \cdot \vec{v}_2 \hat{n} \times \vec{S}_1 \cdot \vec{v}_1 \right) \right) \Bigg\}$$

{DiagSet[3, 9, 58],

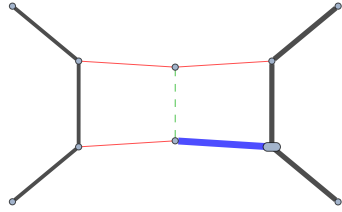

,

$$\begin{aligned} & \frac{1}{r^3} \left( -6 \vec{S}_1 \times \vec{v}_1 \cdot \vec{a}_1 - 6 \vec{S}_1 \times \vec{v}_1 \cdot \vec{a}_2 + 11 \hat{n} \times \vec{S}_1 \cdot \vec{v}_1 \hat{n} \cdot \vec{a}_1 + 8 \hat{n} \times \vec{S}_1 \cdot \vec{v}_1 \hat{n} \cdot \vec{a}_2 - 11 \hat{n} \times \vec{S}_1 \cdot \vec{a}_1 \hat{n} \cdot \vec{v}_1 - 8 \hat{n} \times \vec{S}_1 \cdot \vec{a}_2 \hat{n} \cdot \vec{v}_1 + \pi^2 \right. \\ & \quad \left( \frac{1}{2} \vec{S}_1 \times \vec{v}_1 \cdot \vec{a}_1 + \frac{1}{2} \vec{S}_1 \times \vec{v}_1 \cdot \vec{a}_2 - \frac{3}{4} \hat{n} \times \vec{S}_1 \cdot \vec{v}_1 \hat{n} \cdot \vec{a}_1 - \frac{3}{4} \hat{n} \times \vec{S}_1 \cdot \vec{v}_1 \hat{n} \cdot \vec{a}_2 + \frac{3}{4} \hat{n} \times \vec{S}_1 \cdot \vec{a}_1 \hat{n} \cdot \vec{v}_1 + \frac{3}{4} \hat{n} \times \vec{S}_1 \cdot \vec{a}_2 \hat{n} \cdot \vec{v}_1 \right) \Big) \\ & m_1 m_2^2 G^3 + \frac{1}{r^4} \left( -4 \hat{n} \times \vec{S}_1 \cdot \vec{v}_1 (\hat{n} \cdot \vec{v}_1)^2 - \frac{19}{2} \hat{n} \times \vec{S}_1 \cdot \vec{v}_2 (\hat{n} \cdot \vec{v}_1)^2 - 2 \vec{S}_1 \times \vec{v}_1 \cdot \vec{v}_2 \hat{n} \cdot \vec{v}_1 + \hat{n} \times \vec{S}_1 \cdot \vec{v}_1 \hat{n} \cdot \vec{v}_2 \hat{n} \cdot \vec{v}_1 - \right. \\ & 19 \hat{n} \times \vec{S}_1 \cdot \vec{v}_2 \hat{n} \cdot \vec{v}_2 \hat{n} \cdot \vec{v}_1 + 23 \hat{n} \times \vec{S}_1 \cdot \vec{v}_1 (\hat{n} \cdot \vec{v}_2)^2 - 15 \vec{S}_1 \times \vec{v}_1 \cdot \vec{v}_2 \hat{n} \cdot \vec{v}_2 + 4 \hat{n} \times \vec{S}_1 \cdot \vec{v}_1 \vec{v}_1 \cdot \vec{v}_1 + \\ & \frac{3}{2} \hat{n} \times \vec{S}_1 \cdot \vec{v}_2 \vec{v}_1 \cdot \vec{v}_1 + \hat{n} \times \vec{S}_1 \cdot \vec{v}_1 \vec{v}_1 \cdot \vec{v}_2 + 3 \hat{n} \times \vec{S}_1 \cdot \vec{v}_2 \vec{v}_1 \cdot \vec{v}_2 - 7 \hat{n} \times \vec{S}_1 \cdot \vec{v}_1 \vec{v}_2 \cdot \vec{v}_2 + \\ & \pi^2 \left( \frac{15}{16} \hat{n} \times \vec{S}_1 \cdot \vec{v}_1 (\hat{n} \cdot \vec{v}_1)^2 + \frac{15}{32} \hat{n} \times \vec{S}_1 \cdot \vec{v}_2 (\hat{n} \cdot \vec{v}_1)^2 + \frac{15}{16} \hat{n} \times \vec{S}_1 \cdot \vec{v}_1 \hat{n} \cdot \vec{v}_2 \hat{n} \cdot \vec{v}_1 + \right. \\ & \frac{15}{8} \hat{n} \times \vec{S}_1 \cdot \vec{v}_2 \hat{n} \cdot \vec{v}_2 \hat{n} \cdot \vec{v}_1 - \frac{45}{16} \hat{n} \times \vec{S}_1 \cdot \vec{v}_1 (\hat{n} \cdot \vec{v}_2)^2 + \frac{3}{2} \vec{S}_1 \times \vec{v}_1 \cdot \vec{v}_2 \hat{n} \cdot \vec{v}_2 - \frac{3}{16} \hat{n} \times \vec{S}_1 \cdot \vec{v}_1 \vec{v}_1 \cdot \vec{v}_1 - \\ & \left. \frac{3}{32} \hat{n} \times \vec{S}_1 \cdot \vec{v}_2 \vec{v}_1 \cdot \vec{v}_1 - \frac{3}{16} \hat{n} \times \vec{S}_1 \cdot \vec{v}_1 \vec{v}_1 \cdot \vec{v}_2 - \frac{3}{8} \hat{n} \times \vec{S}_1 \cdot \vec{v}_2 \vec{v}_1 \cdot \vec{v}_2 + \frac{9}{16} \hat{n} \times \vec{S}_1 \cdot \vec{v}_1 \vec{v}_2 \cdot \vec{v}_2 \right) \Big) m_1 m_2^2 G^3 \Big\} \end{aligned}$$

{DiagSet[3, 9, 59],

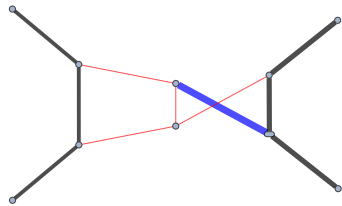

,

$$\begin{aligned} & \frac{1}{r^3} \left( \frac{1}{\vec{S}_1 \times \vec{v}_1 \cdot \vec{v}_2 + \vec{S}_1 \times \vec{a}_1 \cdot \vec{v}_2 - \vec{S}_1 \times \vec{v}_1 \cdot \vec{a}_1 + 7 \hat{n} \times \vec{S}_1 \cdot \vec{v}_1 \hat{n} \cdot \vec{a}_1 - 2 \hat{n} \times \vec{S}_1 \cdot \vec{v}_2 \hat{n} \cdot \vec{a}_1 + 7 \hat{n} \times \vec{S}_1 \cdot \vec{v}_1 \hat{n} \cdot \vec{v}_1 - 2 \hat{n} \times \vec{S}_1 \cdot \vec{v}_2 \hat{n} \cdot \vec{v}_1 - \right. \\ & 3 \hat{n} \times \vec{S}_1 \cdot \vec{v}_1 \hat{n} \cdot \vec{v}_2 - 3 \hat{n} \times \vec{S}_1 \cdot \vec{a}_1 \hat{n} \cdot \vec{v}_2 + \pi^2 \left( -\frac{1}{4} \vec{S}_1 \times \vec{v}_1 \cdot \vec{v}_2 - \frac{1}{4} \vec{S}_1 \times \vec{a}_1 \cdot \vec{v}_2 + \frac{1}{4} \vec{S}_1 \times \vec{v}_1 \cdot \vec{a}_1 - \frac{9}{8} \hat{n} \times \vec{S}_1 \cdot \vec{v}_1 \hat{n} \cdot \vec{a}_1 - \right. \\ & \left. \frac{3}{2} \hat{n} \times \vec{S}_1 \cdot \vec{v}_1 \hat{n} \cdot \vec{v}_1 - \frac{3}{8} \hat{n} \times \vec{S}_1 \cdot \vec{a}_1 \hat{n} \cdot \vec{v}_1 + \frac{3}{4} \hat{n} \times \vec{S}_1 \cdot \vec{v}_1 \hat{n} \cdot \vec{v}_2 + \frac{3}{4} \hat{n} \times \vec{S}_1 \cdot \vec{a}_1 \hat{n} \cdot \vec{v}_2 \right) \Big) m_1 m_2^2 G^3 + \\ & \frac{1}{r^4} \left( -\frac{13}{4} \hat{n} \times \vec{S}_1 \cdot \vec{v}_1 (\hat{n} \cdot \vec{v}_1)^2 + \frac{3}{4} \hat{n} \times \vec{S}_1 \cdot \vec{v}_2 (\hat{n} \cdot \vec{v}_1)^2 - 9 \vec{S}_1 \times \vec{v}_1 \cdot \vec{v}_2 \hat{n} \cdot \vec{v}_1 + \frac{93}{2} \hat{n} \times \vec{S}_1 \cdot \vec{v}_1 \hat{n} \cdot \vec{v}_2 \hat{n} \cdot \vec{v}_1 - \right. \\ & \frac{5}{2} \hat{n} \times \vec{S}_1 \cdot \vec{v}_2 \hat{n} \cdot \vec{v}_2 \hat{n} \cdot \vec{v}_1 - \frac{25}{4} \hat{n} \times \vec{S}_1 \cdot \vec{v}_1 (\hat{n} \cdot \vec{v}_2)^2 + 2 \vec{S}_1 \times \vec{v}_1 \cdot \vec{v}_2 \hat{n} \cdot \vec{v}_2 + \frac{1}{4} \hat{n} \times \vec{S}_1 \cdot \vec{v}_1 \vec{v}_1 \cdot \vec{v}_1 + \\ & \frac{1}{4} \hat{n} \times \vec{S}_1 \cdot \vec{v}_2 \vec{v}_1 \cdot \vec{v}_1 - \frac{17}{2} \hat{n} \times \vec{S}_1 \cdot \vec{v}_1 \vec{v}_1 \cdot \vec{v}_2 - \frac{3}{2} \hat{n} \times \vec{S}_1 \cdot \vec{v}_2 \vec{v}_1 \cdot \vec{v}_2 + \frac{5}{4} \hat{n} \times \vec{S}_1 \cdot \vec{v}_1 \vec{v}_2 \cdot \vec{v}_2 + \\ & \pi^2 \left( \frac{105}{64} \hat{n} \times \vec{S}_1 \cdot \vec{v}_1 (\hat{n} \cdot \vec{v}_1)^2 + \frac{45}{64} \hat{n} \times \vec{S}_1 \cdot \vec{v}_2 (\hat{n} \cdot \vec{v}_1)^2 + \frac{9}{4} \vec{S}_1 \times \vec{v}_1 \cdot \vec{v}_2 \hat{n} \cdot \vec{v}_1 - \frac{315}{32} \hat{n} \times \vec{S}_1 \cdot \vec{v}_1 \hat{n} \cdot \vec{v}_2 \hat{n} \cdot \vec{v}_1 - \right. \\ & \frac{15}{32} \hat{n} \times \vec{S}_1 \cdot \vec{v}_2 \hat{n} \cdot \vec{v}_2 \hat{n} \cdot \vec{v}_1 + \frac{105}{64} \hat{n} \times \vec{S}_1 \cdot \vec{v}_1 (\hat{n} \cdot \vec{v}_2)^2 - \frac{3}{4} \vec{S}_1 \times \vec{v}_1 \cdot \vec{v}_2 \hat{n} \cdot \vec{v}_2 - \frac{21}{64} \hat{n} \times \vec{S}_1 \cdot \vec{v}_1 \vec{v}_1 \cdot \vec{v}_1 - \\ & \left. \frac{9}{64} \hat{n} \times \vec{S}_1 \cdot \vec{v}_2 \vec{v}_1 \cdot \vec{v}_1 + \frac{63}{32} \hat{n} \times \vec{S}_1 \cdot \vec{v}_1 \vec{v}_1 \cdot \vec{v}_2 + \frac{3}{32} \hat{n} \times \vec{S}_1 \cdot \vec{v}_2 \vec{v}_1 \cdot \vec{v}_2 - \frac{21}{64} \hat{n} \times \vec{S}_1 \cdot \vec{v}_1 \vec{v}_2 \cdot \vec{v}_2 \right) \Big) m_1 m_2^2 G^3 \Big\} \end{aligned}$$

{DiagSet[3, 9, 60],

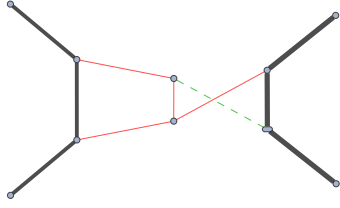

,

$$\frac{\left( \hat{n} \times \vec{S}_1 \cdot \vec{a}_1 + \pi^2 \left( -\frac{1}{4} \hat{n} \times \vec{S}_1 \cdot \vec{a}_1 - \frac{1}{4} \hat{n} \times \vec{S}_1 \cdot \vec{a}_2 \right) + \hat{n} \times \vec{S}_1 \cdot \vec{a}_2 \right) m_1 m_2^2 G^3}{r^2} + \frac{1}{r^3} \left( \frac{1}{\vec{S}_1 \times \vec{v}_1 \cdot \vec{v}_2} - \vec{S}_1 \times \vec{a}_1 \cdot \vec{v}_2 - \vec{S}_1 \times \vec{v}_1 \cdot \vec{a}_1 + 2 \vec{S}_1 \times \vec{v}_2 \cdot \vec{a}_2 + 2 \hat{n} \times \vec{S}_1 \cdot \vec{v}_1 \hat{n} \cdot \vec{a}_1 - 4 \hat{n} \times \vec{S}_1 \cdot \vec{v}_1 \hat{n} \cdot \vec{a}_2 - 3 \hat{n} \times \vec{S}_1 \cdot \vec{v}_2 \hat{n} \cdot \vec{a}_2 - \right. \\ \left. 4 \hat{n} \times \vec{S}_1 \cdot \vec{v}_1 \hat{n} \cdot \vec{v}_1 + 3 \hat{n} \times \vec{S}_1 \cdot \vec{v}_2 \hat{n} \cdot \vec{v}_1 - \hat{n} \times \vec{S}_1 \cdot \vec{a}_1 \hat{n} \cdot \vec{v}_1 - 2 \hat{n} \times \vec{S}_1 \cdot \vec{a}_2 \hat{n} \cdot \vec{v}_1 - 6 \hat{n} \times \vec{S}_1 \cdot \vec{v}_1 \hat{n} \cdot \vec{v}_2 + 5 \hat{n} \times \vec{S}_1 \cdot \vec{v}_2 \hat{n} \cdot \vec{v}_2 + \right. \\ \left. 3 \hat{n} \times \vec{S}_1 \cdot \vec{a}_1 \hat{n} \cdot \vec{v}_2 + 3 \hat{n} \times \vec{S}_1 \cdot \vec{a}_2 \hat{n} \cdot \vec{v}_2 + \pi^2 \left( -\frac{1}{4} \vec{S}_1 \times \vec{v}_1 \cdot \vec{v}_2 + \frac{1}{4} \vec{S}_1 \times \vec{a}_1 \cdot \vec{v}_2 + \frac{1}{4} \vec{S}_1 \times \vec{v}_1 \cdot \vec{a}_1 - \frac{1}{2} \vec{S}_1 \times \vec{v}_2 \cdot \vec{a}_2 - \right. \right. \\ \left. \frac{3}{8} \hat{n} \times \vec{S}_1 \cdot \vec{v}_1 \hat{n} \cdot \vec{a}_1 + \frac{3}{4} \hat{n} \times \vec{S}_1 \cdot \vec{v}_1 \hat{n} \cdot \vec{a}_2 + \frac{3}{4} \hat{n} \times \vec{S}_1 \cdot \vec{v}_2 \hat{n} \cdot \vec{a}_2 + \frac{3}{4} \hat{n} \times \vec{S}_1 \cdot \vec{v}_1 \hat{n} \cdot \vec{v}_1 + \frac{3}{8} \hat{n} \times \vec{S}_1 \cdot \vec{a}_1 \hat{n} \cdot \vec{v}_1 + \right. \\ \left. \frac{3}{4} \hat{n} \times \vec{S}_1 \cdot \vec{a}_2 \hat{n} \cdot \vec{v}_1 + \frac{3}{4} \hat{n} \times \vec{S}_1 \cdot \vec{v}_1 \hat{n} \cdot \vec{v}_2 - \frac{3}{4} \hat{n} \times \vec{S}_1 \cdot \vec{v}_2 \hat{n} \cdot \vec{v}_2 - \frac{3}{4} \hat{n} \times \vec{S}_1 \cdot \vec{a}_1 \hat{n} \cdot \vec{v}_2 - \frac{3}{4} \hat{n} \times \vec{S}_1 \cdot \vec{a}_2 \hat{n} \cdot \vec{v}_2 \right) \Big) m_1 m_2^2 G^3 + \\ \frac{1}{r^4} \left( -\frac{1}{4} \hat{n} \times \vec{S}_1 \cdot \vec{v}_1 (\hat{n} \cdot \vec{v}_1)^2 - \frac{3}{4} \hat{n} \times \vec{S}_1 \cdot \vec{v}_2 (\hat{n} \cdot \vec{v}_1)^2 + 2 \vec{S}_1 \times \vec{v}_1 \cdot \vec{v}_2 \hat{n} \cdot \vec{v}_1 - \frac{23}{2} \hat{n} \times \vec{S}_1 \cdot \vec{v}_1 \hat{n} \cdot \vec{v}_2 \hat{n} \cdot \vec{v}_1 - \right. \\ \left. \frac{13}{2} \hat{n} \times \vec{S}_1 \cdot \vec{v}_2 \hat{n} \cdot \vec{v}_2 \hat{n} \cdot \vec{v}_1 - \frac{83}{4} \hat{n} \times \vec{S}_1 \cdot \vec{v}_1 (\hat{n} \cdot \vec{v}_2)^2 + \frac{9}{2} \hat{n} \times \vec{S}_1 \cdot \vec{v}_2 (\hat{n} \cdot \vec{v}_2)^2 + 5 \vec{S}_1 \times \vec{v}_1 \cdot \vec{v}_2 \hat{n} \cdot \vec{v}_2 + \right. \\ \left. \frac{5}{4} \hat{n} \times \vec{S}_1 \cdot \vec{v}_1 \vec{v}_1 \cdot \vec{v}_1 - \frac{9}{4} \hat{n} \times \vec{S}_1 \cdot \vec{v}_2 \vec{v}_1 \cdot \vec{v}_1 + \frac{7}{2} \hat{n} \times \vec{S}_1 \cdot \vec{v}_1 \vec{v}_1 \cdot \vec{v}_2 + \frac{5}{2} \hat{n} \times \vec{S}_1 \cdot \vec{v}_2 \vec{v}_1 \cdot \vec{v}_2 + \right. \\ \left. \frac{7}{4} \hat{n} \times \vec{S}_1 \cdot \vec{v}_1 \vec{v}_2 \cdot \vec{v}_2 + \frac{3}{2} \hat{n} \times \vec{S}_1 \cdot \vec{v}_2 \vec{v}_2 \cdot \vec{v}_2 + \pi^2 \left( -\frac{15}{64} \hat{n} \times \vec{S}_1 \cdot \vec{v}_1 (\hat{n} \cdot \vec{v}_1)^2 - \frac{45}{64} \hat{n} \times \vec{S}_1 \cdot \vec{v}_2 (\hat{n} \cdot \vec{v}_1)^2 - \right. \right. \\ \left. \frac{3}{4} \vec{S}_1 \times \vec{v}_1 \cdot \vec{v}_2 \hat{n} \cdot \vec{v}_1 + \frac{75}{32} \hat{n} \times \vec{S}_1 \cdot \vec{v}_1 \hat{n} \cdot \vec{v}_2 \hat{n} \cdot \vec{v}_1 + \frac{75}{32} \hat{n} \times \vec{S}_1 \cdot \vec{v}_2 \hat{n} \cdot \vec{v}_2 \hat{n} \cdot \vec{v}_1 + \frac{195}{64} \hat{n} \times \vec{S}_1 \cdot \vec{v}_1 (\hat{n} \cdot \vec{v}_2)^2 - \right. \\ \left. \frac{15}{32} \hat{n} \times \vec{S}_1 \cdot \vec{v}_2 (\hat{n} \cdot \vec{v}_2)^2 - \frac{3}{4} \vec{S}_1 \times \vec{v}_1 \cdot \vec{v}_2 \hat{n} \cdot \vec{v}_2 + \frac{3}{64} \hat{n} \times \vec{S}_1 \cdot \vec{v}_1 \vec{v}_1 \cdot \vec{v}_1 + \frac{9}{64} \hat{n} \times \vec{S}_1 \cdot \vec{v}_2 \vec{v}_1 \cdot \vec{v}_1 - \right. \\ \left. \frac{15}{32} \hat{n} \times \vec{S}_1 \cdot \vec{v}_1 \vec{v}_1 \cdot \vec{v}_2 - \frac{15}{32} \hat{n} \times \vec{S}_1 \cdot \vec{v}_2 \vec{v}_1 \cdot \vec{v}_2 - \frac{39}{64} \hat{n} \times \vec{S}_1 \cdot \vec{v}_1 \vec{v}_2 \cdot \vec{v}_2 + \frac{3}{32} \hat{n} \times \vec{S}_1 \cdot \vec{v}_2 \vec{v}_2 \cdot \vec{v}_2 \right) \Big) m_1 m_2^2 G^3 \Big\}$$

{DiagSet[3, 9, 61],

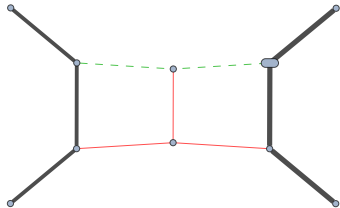

,

$$\frac{1}{r^3} \left( -12 \vec{S}_1 \times \vec{v}_2 \cdot \vec{a}_2 + 4 \hat{n} \times \vec{S}_1 \cdot \vec{v}_1 \hat{n} \cdot \vec{a}_2 + 16 \hat{n} \times \vec{S}_1 \cdot \vec{v}_2 \hat{n} \cdot \vec{a}_2 + 20 \hat{n} \times \vec{S}_1 \cdot \vec{v}_2 \hat{n} \cdot \vec{v}_1 + 20 \hat{n} \times \vec{S}_1 \cdot \vec{a}_2 \hat{n} \cdot \vec{v}_1 + \right. \\ \left. 4 \hat{n} \times \vec{S}_1 \cdot \vec{v}_1 \hat{n} \cdot \vec{v}_2 - 28 \hat{n} \times \vec{S}_1 \cdot \vec{v}_2 \hat{n} \cdot \vec{v}_2 - 44 \hat{n} \times \vec{S}_1 \cdot \vec{a}_2 \hat{n} \cdot \vec{v}_2 + \pi^2 \left( \frac{1}{2} \vec{S}_1 \times \vec{v}_1 \cdot \vec{v}_2 + \frac{1}{2} \vec{S}_1 \times \vec{v}_1 \cdot \vec{a}_2 + 2 \vec{S}_1 \times \vec{v}_2 \cdot \vec{a}_2 - \right. \right. \\ \left. \frac{3}{2} \hat{n} \times \vec{S}_1 \cdot \vec{v}_1 \hat{n} \cdot \vec{a}_2 - 3 \hat{n} \times \vec{S}_1 \cdot \vec{v}_2 \hat{n} \cdot \vec{a}_2 - \frac{3}{2} \hat{n} \times \vec{S}_1 \cdot \vec{v}_1 \hat{n} \cdot \vec{v}_2 + 3 \hat{n} \times \vec{S}_1 \cdot \vec{a}_2 \hat{n} \cdot \vec{v}_2 \right) \Big) m_1 m_2^2 G^3 + \frac{1}{r^4} \\ \left( -75 \hat{n} \times \vec{S}_1 \cdot \vec{v}_2 (\hat{n} \cdot \vec{v}_1)^2 - 28 \vec{S}_1 \times \vec{v}_1 \cdot \vec{v}_2 \hat{n} \cdot \vec{v}_1 + 6 \hat{n} \times \vec{S}_1 \cdot \vec{v}_1 \hat{n} \cdot \vec{v}_2 \hat{n} \cdot \vec{v}_1 + 190 \hat{n} \times \vec{S}_1 \cdot \vec{v}_2 \hat{n} \cdot \vec{v}_2 \hat{n} \cdot \vec{v}_1 + \right. \\ \left. 39 \hat{n} \times \vec{S}_1 \cdot \vec{v}_1 (\hat{n} \cdot \vec{v}_2)^2 - 95 \hat{n} \times \vec{S}_1 \cdot \vec{v}_2 (\hat{n} \cdot \vec{v}_2)^2 + 12 \vec{S}_1 \times \vec{v}_1 \cdot \vec{v}_2 \hat{n} \cdot \vec{v}_2 + 7 \hat{n} \times \vec{S}_1 \cdot \vec{v}_2 \vec{v}_1 \cdot \vec{v}_1 + \right. \\ \left. 2 \hat{n} \times \vec{S}_1 \cdot \vec{v}_1 \vec{v}_1 \cdot \vec{v}_2 - 30 \hat{n} \times \vec{S}_1 \cdot \vec{v}_2 \vec{v}_1 \cdot \vec{v}_2 - 7 \hat{n} \times \vec{S}_1 \cdot \vec{v}_1 \vec{v}_2 \cdot \vec{v}_2 + 3 \hat{n} \times \vec{S}_1 \cdot \vec{v}_2 \vec{v}_2 \cdot \vec{v}_2 + \right. \\ \left. 2 \hat{n} \times \vec{S}_1 \cdot \vec{v}_1 \vec{v}_2 \cdot \vec{v}_2 + 3 \hat{n} \times \vec{S}_1 \cdot \vec{v}_2 \vec{v}_2 \cdot \vec{v}_2 \right) \Big\}$$



$$\pi^2 \left( \frac{15}{16} \hat{n} \times \vec{S}_1 \cdot \vec{v}_2 (\hat{n} \cdot \vec{v}_1)^2 + \frac{15}{8} \hat{n} \times \vec{S}_1 \cdot \vec{v}_1 \hat{n} \cdot \vec{v}_2 \hat{n} \cdot \vec{v}_1 + \frac{15}{8} \hat{n} \times \vec{S}_1 \cdot \vec{v}_2 \hat{n} \cdot \vec{v}_2 \hat{n} \cdot \vec{v}_1 - \right. \\ \left. \frac{135}{16} \hat{n} \times \vec{S}_1 \cdot \vec{v}_1 (\hat{n} \cdot \vec{v}_2)^2 + \frac{15}{16} \hat{n} \times \vec{S}_1 \cdot \vec{v}_2 (\hat{n} \cdot \vec{v}_2)^2 + \frac{15}{4} \vec{S}_1 \times \vec{v}_1 \cdot \vec{v}_2 \hat{n} \cdot \vec{v}_2 - \frac{3}{16} \hat{n} \times \vec{S}_1 \cdot \vec{v}_2 \vec{v}_1 \cdot \vec{v}_1 - \right. \\ \left. \frac{3}{8} \hat{n} \times \vec{S}_1 \cdot \vec{v}_1 \vec{v}_1 \cdot \vec{v}_2 - \frac{3}{8} \hat{n} \times \vec{S}_1 \cdot \vec{v}_2 \vec{v}_1 \cdot \vec{v}_2 + \frac{27}{16} \hat{n} \times \vec{S}_1 \cdot \vec{v}_1 \vec{v}_2 \cdot \vec{v}_2 - \frac{3}{16} \hat{n} \times \vec{S}_1 \cdot \vec{v}_2 \vec{v}_2 \cdot \vec{v}_2 \right) \left. m_1 m_2^2 G^3 \right\}$$

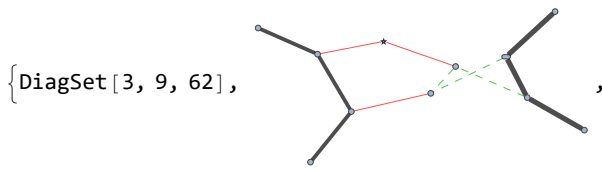

$$\frac{1}{r^3} G^3 m_1 m_2^2 \left( 4 \hat{n} \cdot \vec{a}_1 \hat{n} \times \vec{S}_1 \cdot \vec{v}_2 + \pi^2 \left( -\frac{3}{8} \hat{n} \cdot \vec{a}_1 \hat{n} \times \vec{S}_1 \cdot \vec{v}_2 - \frac{3}{2} \hat{n} \cdot \vec{v}_2 \hat{n} \times \vec{a}_1 \cdot \vec{S}_1 + \frac{5}{8} \vec{a}_1 \times \vec{S}_1 \cdot \vec{v}_2 - \frac{3}{8} \hat{n} \cdot \vec{v}_1 \hat{n} \times \vec{S}_1 \cdot \vec{v}_2 + \right. \right. \\ \left. \left. \frac{3}{2} \hat{n} \cdot \vec{v}_2 \hat{n} \times \vec{S}_1 \cdot \vec{v}_1 - \frac{5}{8} \vec{S}_1 \times \vec{v}_1 \cdot \vec{v}_2 \right) - 2 \vec{a}_1 \times \vec{S}_1 \cdot \vec{v}_2 + 4 \hat{n} \cdot \vec{v}_1 \hat{n} \times \vec{S}_1 \cdot \vec{v}_2 + 2 \vec{S}_1 \times \vec{v}_1 \cdot \vec{v}_2 \right) + \frac{1}{r^4} \\ G^3 m_1 m_2^2 \left( -20 (\hat{n} \cdot \vec{v}_1)^2 \hat{n} \times \vec{S}_1 \cdot \vec{v}_2 - 10 \hat{n} \cdot \vec{v}_1 \vec{S}_1 \times \vec{v}_1 \cdot \vec{v}_2 + 16 \hat{n} \cdot \vec{v}_2 \hat{n} \cdot \vec{v}_1 \hat{n} \times \vec{S}_1 \cdot \vec{v}_2 - 12 (\hat{n} \cdot \vec{v}_2)^2 \hat{n} \times \vec{S}_1 \cdot \vec{v}_1 + \right. \\ \left. 10 \hat{n} \cdot \vec{v}_2 \vec{S}_1 \times \vec{v}_1 \cdot \vec{v}_2 + 4 \vec{v}_1 \cdot \vec{v}_1 \hat{n} \times \vec{S}_1 \cdot \vec{v}_2 - 4 \vec{v}_1 \cdot \vec{v}_2 \hat{n} \times \vec{S}_1 \cdot \vec{v}_2 + 4 \vec{v}_2 \cdot \vec{v}_2 \hat{n} \times \vec{S}_1 \cdot \vec{v}_1 + \pi^2 \left( \frac{15}{8} (\hat{n} \cdot \vec{v}_1)^2 \hat{n} \times \vec{S}_1 \cdot \vec{v}_2 + \right. \right. \\ \left. \left. \frac{9}{4} \hat{n} \cdot \vec{v}_1 \vec{S}_1 \times \vec{v}_1 \cdot \vec{v}_2 - \frac{15}{2} \hat{n} \cdot \vec{v}_2 \hat{n} \cdot \vec{v}_1 \hat{n} \times \vec{S}_1 \cdot \vec{v}_1 - \frac{15}{16} \hat{n} \cdot \vec{v}_2 \hat{n} \cdot \vec{v}_1 \hat{n} \times \vec{S}_1 \cdot \vec{v}_2 + \frac{135}{32} (\hat{n} \cdot \vec{v}_2)^2 \hat{n} \times \vec{S}_1 \cdot \vec{v}_1 - \right. \right. \\ \left. \left. \frac{15}{8} \hat{n} \cdot \vec{v}_2 \vec{S}_1 \times \vec{v}_1 \cdot \vec{v}_2 - \frac{3}{8} \vec{v}_1 \cdot \vec{v}_1 \hat{n} \times \vec{S}_1 \cdot \vec{v}_2 + \frac{3}{2} \vec{v}_1 \cdot \vec{v}_2 \hat{n} \times \vec{S}_1 \cdot \vec{v}_1 + \frac{3}{16} \vec{v}_1 \cdot \vec{v}_2 \hat{n} \times \vec{S}_1 \cdot \vec{v}_2 - \frac{27}{32} \vec{v}_2 \cdot \vec{v}_2 \hat{n} \times \vec{S}_1 \cdot \vec{v}_1 \right) \right) \left. \right\}$$

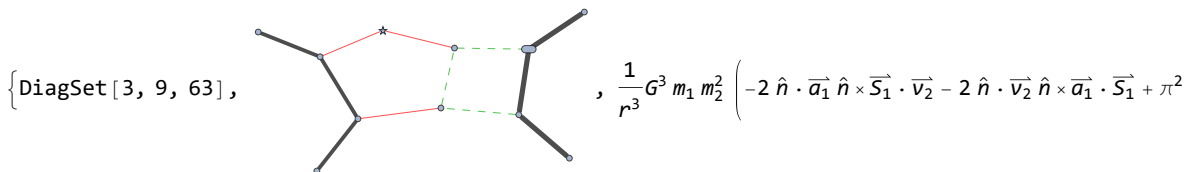

$$\frac{1}{r^3} G^3 m_1 m_2^2 \left( -2 \hat{n} \cdot \vec{a}_1 \hat{n} \times \vec{S}_1 \cdot \vec{v}_2 - 2 \hat{n} \cdot \vec{v}_2 \hat{n} \times \vec{a}_1 \cdot \vec{S}_1 + \pi^2 \left( \frac{3}{8} \hat{n} \cdot \vec{a}_1 \hat{n} \times \vec{S}_1 \cdot \vec{v}_2 - \frac{3}{4} \hat{n} \cdot \vec{v}_2 \hat{n} \times \vec{a}_1 \cdot \vec{S}_1 + \frac{1}{8} \vec{a}_1 \times \vec{S}_1 \cdot \vec{v}_2 + \frac{3}{8} \hat{n} \cdot \vec{v}_1 \hat{n} \times \vec{S}_1 \cdot \vec{v}_2 + \frac{3}{4} \hat{n} \cdot \vec{v}_2 \hat{n} \times \vec{S}_1 \cdot \vec{v}_1 - \frac{1}{8} \vec{S}_1 \times \vec{v}_1 \cdot \vec{v}_2 \right) + \right. \\ \left. 2 \vec{a}_1 \times \vec{S}_1 \cdot \vec{v}_2 - 2 \hat{n} \cdot \vec{v}_1 \hat{n} \times \vec{S}_1 \cdot \vec{v}_2 + 2 \hat{n} \cdot \vec{v}_2 \hat{n} \times \vec{S}_1 \cdot \vec{v}_1 - 2 \vec{S}_1 \times \vec{v}_1 \cdot \vec{v}_2 \right) + \frac{1}{r^4} \\ G^3 m_1 m_2^2 \left( 10 (\hat{n} \cdot \vec{v}_1)^2 \hat{n} \times \vec{S}_1 \cdot \vec{v}_2 + 8 \hat{n} \cdot \vec{v}_1 \vec{S}_1 \times \vec{v}_1 \cdot \vec{v}_2 - 10 \hat{n} \cdot \vec{v}_2 \hat{n} \cdot \vec{v}_1 \hat{n} \times \vec{S}_1 \cdot \vec{v}_1 - 9 \hat{n} \cdot \vec{v}_2 \hat{n} \cdot \vec{v}_1 \hat{n} \times \vec{S}_1 \cdot \vec{v}_2 + \right. \\ \left. \frac{33}{2} (\hat{n} \cdot \vec{v}_2)^2 \hat{n} \times \vec{S}_1 \cdot \vec{v}_1 - 8 \hat{n} \cdot \vec{v}_2 \vec{S}_1 \times \vec{v}_1 \cdot \vec{v}_2 - 2 \vec{v}_1 \cdot \vec{v}_1 \hat{n} \times \vec{S}_1 \cdot \vec{v}_2 + 2 \vec{v}_1 \cdot \vec{v}_2 \hat{n} \times \vec{S}_1 \cdot \vec{v}_1 + \vec{v}_1 \cdot \vec{v}_2 \hat{n} \times \vec{S}_1 \cdot \vec{v}_2 + \right. \\ \left. \pi^2 \left( -\frac{15}{8} (\hat{n} \cdot \vec{v}_1)^2 \hat{n} \times \vec{S}_1 \cdot \vec{v}_2 - \frac{15}{4} \hat{n} \cdot \vec{v}_2 \hat{n} \cdot \vec{v}_1 \hat{n} \times \vec{S}_1 \cdot \vec{v}_1 + \frac{15}{8} \hat{n} \cdot \vec{v}_2 \hat{n} \cdot \vec{v}_1 \hat{n} \times \vec{S}_1 \cdot \vec{v}_2 + \frac{3}{8} \hat{n} \cdot \vec{v}_2 \vec{S}_1 \times \vec{v}_1 \cdot \vec{v}_2 + \right. \right. \\ \left. \left. \frac{3}{8} \vec{v}_1 \cdot \vec{v}_1 \hat{n} \times \vec{S}_1 \cdot \vec{v}_2 + \frac{3}{4} \vec{v}_1 \cdot \vec{v}_2 \hat{n} \times \vec{S}_1 \cdot \vec{v}_1 - \frac{3}{8} \vec{v}_1 \cdot \vec{v}_2 \hat{n} \times \vec{S}_1 \cdot \vec{v}_2 \right) - \frac{5}{2} \vec{v}_2 \cdot \vec{v}_2 \hat{n} \times \vec{S}_1 \cdot \vec{v}_1 \right) \left. \right\}$$

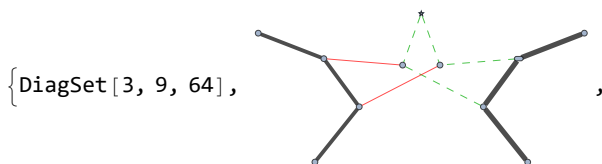

$$\left( \frac{6 \hat{n} \times \vec{a}_1 \cdot \vec{S}_1 - \frac{1}{2} \pi^2 \hat{n} \times \vec{a}_1 \cdot \vec{S}_1}{r^2} \right) m_1 m_2^2 G^3 + \frac{1}{r^3} \left( -24 \vec{S}_1 \times \vec{v}_1 \cdot \vec{v}_2 + 18 \vec{a}_1 \times \vec{S}_1 \cdot \vec{v}_1 - 30 \vec{a}_1 \times \vec{S}_1 \cdot \vec{v}_2 - 26 \hat{n} \times \vec{S}_1 \cdot \vec{v}_1 \hat{n} \cdot \vec{a}_1 + \right. \\ \left. 34 \hat{n} \times \vec{S}_1 \cdot \vec{v}_2 \hat{n} \cdot \vec{a}_1 + 8 \hat{n} \times \vec{S}_1 \cdot \vec{v}_1 \hat{n} \cdot \vec{v}_1 - 34 \hat{n} \times \vec{S}_1 \cdot \vec{v}_2 \hat{n} \cdot \vec{v}_1 - 36 \hat{n} \times \vec{a}_1 \cdot \vec{S}_1 \hat{n} \cdot \vec{v}_1 + 26 \hat{n} \times \vec{S}_1 \cdot \vec{v}_1 \hat{n} \cdot \vec{v}_2 + \right.$$

$$\begin{aligned}
& 44 \hat{n} \times \vec{a}_1 \cdot \vec{S}_1 \hat{n} \cdot \vec{v}_2 + \pi^2 \left( \frac{3}{2} \vec{S}_1 \times \vec{v}_1 \cdot \vec{v}_2 - \frac{3}{4} \vec{a}_1 \times \vec{S}_1 \cdot \vec{v}_1 + 2 \vec{a}_1 \times \vec{S}_1 \cdot \vec{v}_2 + \frac{3}{4} \hat{n} \times \vec{S}_1 \cdot \vec{v}_1 \hat{n} \cdot \vec{a}_1 - 3 \hat{n} \times \vec{S}_1 \cdot \vec{v}_2 \hat{n} \cdot \vec{a}_1 - \right. \\
& \quad \left. \frac{3}{4} \hat{n} \times \vec{S}_1 \cdot \vec{v}_1 \hat{n} \cdot \vec{v}_1 + 3 \hat{n} \times \vec{S}_1 \cdot \vec{v}_2 \hat{n} \cdot \vec{v}_1 + \frac{3}{2} \hat{n} \times \vec{a}_1 \cdot \vec{S}_1 \hat{n} \cdot \vec{v}_1 - \frac{3}{2} \hat{n} \times \vec{S}_1 \cdot \vec{v}_1 \hat{n} \cdot \vec{v}_2 - 3 \hat{n} \times \vec{a}_1 \cdot \vec{S}_1 \hat{n} \cdot \vec{v}_2 \right) \Big) m_1 m_2^2 G^3 + \\
& \frac{1}{r^4} \left( -\frac{33}{2} \hat{n} \times \vec{S}_1 \cdot \vec{v}_1 (\hat{n} \cdot \vec{v}_1)^2 + 53 \hat{n} \times \vec{S}_1 \cdot \vec{v}_2 (\hat{n} \cdot \vec{v}_1)^2 + 30 \vec{S}_1 \times \vec{v}_1 \cdot \vec{v}_2 \hat{n} \cdot \vec{v}_1 - 56 \hat{n} \times \vec{S}_1 \cdot \vec{v}_1 \hat{n} \cdot \vec{v}_2 \hat{n} \cdot \vec{v}_1 - \right. \\
& \quad 67 \hat{n} \times \vec{S}_1 \cdot \vec{v}_2 \hat{n} \cdot \vec{v}_2 \hat{n} \cdot \vec{v}_1 + \frac{47}{2} \hat{n} \times \vec{S}_1 \cdot \vec{v}_1 (\hat{n} \cdot \vec{v}_2)^2 - 22 \vec{S}_1 \times \vec{v}_1 \cdot \vec{v}_2 \hat{n} \cdot \vec{v}_2 + \frac{5}{2} \hat{n} \times \vec{S}_1 \cdot \vec{v}_1 \vec{v}_1 \cdot \vec{v}_1 - \\
& \quad 17 \hat{n} \times \vec{S}_1 \cdot \vec{v}_2 \vec{v}_1 \cdot \vec{v}_1 + 16 \hat{n} \times \vec{S}_1 \cdot \vec{v}_1 \vec{v}_1 \cdot \vec{v}_2 + 15 \hat{n} \times \vec{S}_1 \cdot \vec{v}_2 \vec{v}_1 \cdot \vec{v}_2 - \frac{19}{2} \hat{n} \times \vec{S}_1 \cdot \vec{v}_1 \vec{v}_2 \cdot \vec{v}_2 + \\
& \quad \pi^2 \left( \frac{45}{32} \hat{n} \times \vec{S}_1 \cdot \vec{v}_1 (\hat{n} \cdot \vec{v}_1)^2 - \frac{75}{16} \hat{n} \times \vec{S}_1 \cdot \vec{v}_2 (\hat{n} \cdot \vec{v}_1)^2 - 3 \vec{S}_1 \times \vec{v}_1 \cdot \vec{v}_2 \hat{n} \cdot \vec{v}_1 + \frac{45}{8} \hat{n} \times \vec{S}_1 \cdot \vec{v}_1 \hat{n} \cdot \vec{v}_2 \hat{n} \cdot \vec{v}_1 + \right. \\
& \quad \frac{105}{16} \hat{n} \times \vec{S}_1 \cdot \vec{v}_2 \hat{n} \cdot \vec{v}_2 \hat{n} \cdot \vec{v}_1 - \frac{75}{32} \hat{n} \times \vec{S}_1 \cdot \vec{v}_1 (\hat{n} \cdot \vec{v}_2)^2 + \frac{9}{4} \vec{S}_1 \times \vec{v}_1 \cdot \vec{v}_2 \hat{n} \cdot \vec{v}_2 - \frac{9}{32} \hat{n} \times \vec{S}_1 \cdot \vec{v}_1 \vec{v}_1 \cdot \vec{v}_1 + \\
& \quad \left. \frac{15}{16} \hat{n} \times \vec{S}_1 \cdot \vec{v}_2 \vec{v}_1 \cdot \vec{v}_1 - \frac{9}{8} \hat{n} \times \vec{S}_1 \cdot \vec{v}_1 \vec{v}_1 \cdot \vec{v}_2 - \frac{21}{16} \hat{n} \times \vec{S}_1 \cdot \vec{v}_2 \vec{v}_1 \cdot \vec{v}_2 + \frac{15}{32} \hat{n} \times \vec{S}_1 \cdot \vec{v}_1 \vec{v}_2 \cdot \vec{v}_2 \right) \Big) m_1 m_2^2 G^3 \Big\}
\end{aligned}$$

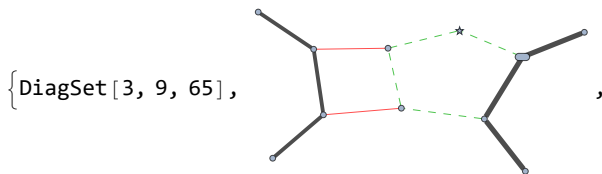

$$\begin{aligned}
& \frac{1}{r^3} G^3 m_1 m_2^2 \left( 8 \hat{n} \cdot \vec{a}_1 \hat{n} \times \vec{S}_1 \cdot \vec{v}_1 + 8 \hat{n} \cdot \vec{v}_1 \hat{n} \times \vec{a}_1 \cdot \vec{S}_1 + \pi^2 \left( -\frac{15}{8} \hat{n} \cdot \vec{a}_1 \hat{n} \times \vec{S}_1 \cdot \vec{v}_1 - \frac{3}{4} \hat{n} \cdot \vec{v}_1 \hat{n} \times \vec{a}_1 \cdot \vec{S}_1 + \right. \right. \\
& \quad \left. \frac{7}{8} \vec{a}_1 \times \vec{S}_1 \cdot \vec{v}_1 - \frac{15}{8} \hat{n} \cdot \vec{v}_1 \hat{n} \times \vec{S}_1 \cdot \vec{v}_1 + 3 \hat{n} \cdot \vec{v}_2 \hat{n} \times \vec{S}_1 \cdot \vec{v}_1 - \left( \frac{1}{\vec{S}_1 \times \vec{v}_1 \cdot \vec{v}_2} \right) \right) - 8 \vec{a}_1 \times \vec{S}_1 \cdot \vec{v}_1 - \\
& \quad \left. 18 \hat{n} \cdot \vec{v}_1 \hat{n} \times \vec{S}_1 \cdot \vec{v}_1 + 18 \hat{n} \cdot \vec{v}_2 \hat{n} \times \vec{S}_1 \cdot \vec{v}_1 - 6 \vec{S}_1 \times \vec{v}_1 \cdot \vec{v}_2 \right) + \frac{G^3 m_1 m_2^2 \left( -\pi^2 \hat{n} \times \vec{a}_1 \cdot \vec{S}_1 - 6 \hat{n} \times \vec{a}_1 \cdot \vec{S}_1 \right)}{r^2} + \\
& \frac{1}{r^4} G^3 m_1 m_2^2 \left( \frac{11}{2} (\hat{n} \cdot \vec{v}_1)^2 \hat{n} \times \vec{S}_1 \cdot \vec{v}_1 - \frac{7}{2} \vec{v}_1 \cdot \vec{v}_1 \hat{n} \times \vec{S}_1 \cdot \vec{v}_1 + \pi^2 \left( \frac{75}{32} (\hat{n} \cdot \vec{v}_1)^2 \hat{n} \times \vec{S}_1 \cdot \vec{v}_1 + \right. \right. \\
& \quad \left. \frac{9}{8} \hat{n} \cdot \vec{v}_1 \vec{S}_1 \times \vec{v}_1 \cdot \vec{v}_2 - \frac{45}{8} \hat{n} \cdot \vec{v}_2 \hat{n} \cdot \vec{v}_1 \hat{n} \times \vec{S}_1 \cdot \vec{v}_1 - \frac{15}{32} \vec{v}_1 \cdot \vec{v}_1 \hat{n} \times \vec{S}_1 \cdot \vec{v}_1 + \frac{9}{8} \vec{v}_1 \cdot \vec{v}_2 \hat{n} \times \vec{S}_1 \cdot \vec{v}_1 \right) \Big) \Big\}
\end{aligned}$$

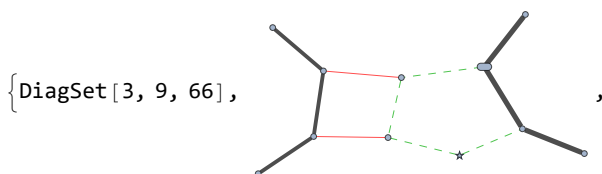

$$\begin{aligned}
& \frac{1}{r^3} G^3 m_1 m_2^2 \left( -2 \hat{n} \cdot \vec{a}_1 \hat{n} \times \vec{S}_1 \cdot \vec{v}_1 - 12 \hat{n} \cdot \vec{v}_1 \hat{n} \times \vec{a}_1 \cdot \vec{S}_1 + 12 \hat{n} \cdot \vec{v}_2 \hat{n} \times \vec{a}_1 \cdot \vec{S}_1 + \right. \\
& \quad \pi^2 \left( -\frac{27}{8} \hat{n} \cdot \vec{a}_1 \hat{n} \times \vec{S}_1 \cdot \vec{v}_1 - \frac{27}{4} \hat{n} \cdot \vec{v}_1 \hat{n} \times \vec{a}_1 \cdot \vec{S}_1 + \frac{9}{2} \hat{n} \cdot \vec{v}_2 \hat{n} \times \vec{a}_1 \cdot \vec{S}_1 + \frac{27}{8} \vec{a}_1 \times \vec{S}_1 \cdot \vec{v}_1 - \right. \\
& \quad \left. \frac{3}{2} \vec{a}_1 \times \vec{S}_1 \cdot \vec{v}_2 + \frac{9}{8} \hat{n} \cdot \vec{v}_1 \hat{n} \times \vec{S}_1 \cdot \vec{v}_1 \right) + 2 \vec{a}_1 \times \vec{S}_1 \cdot \vec{v}_1 - 4 \vec{a}_1 \times \vec{S}_1 \cdot \vec{v}_2 + 2 \hat{n} \cdot \vec{v}_1 \hat{n} \times \vec{S}_1 \cdot \vec{v}_1 \Big) + \\
& \frac{G^3 m_1 m_2^2 \left( \frac{3}{2} \pi^2 \hat{n} \times \vec{a}_1 \cdot \vec{S}_1 + 4 \hat{n} \times \vec{a}_1 \cdot \vec{S}_1 \right)}{r^2} + \frac{1}{r^4} G^3 m_1 m_2^2 \left( -6 (\hat{n} \cdot \vec{v}_1)^2 \hat{n} \times \vec{S}_1 \cdot \vec{v}_1 - 2 \hat{n} \cdot \vec{v}_1 \vec{S}_1 \times \vec{v}_1 \cdot \vec{v}_2 + \right. \\
& \quad \left. 10 \hat{n} \cdot \vec{v}_2 \hat{n} \cdot \vec{v}_1 \hat{n} \times \vec{S}_1 \cdot \vec{v}_1 + 2 \vec{v}_1 \cdot \vec{v}_1 \hat{n} \times \vec{S}_1 \cdot \vec{v}_1 - 2 \vec{v}_1 \cdot \vec{v}_2 \hat{n} \times \vec{S}_1 \cdot \vec{v}_1 + \pi^2 \left( -\frac{45}{16} (\hat{n} \cdot \vec{v}_1)^2 \hat{n} \times \vec{S}_1 \cdot \vec{v}_1 - \right. \right.
\end{aligned}$$

$$\frac{9}{8} \hat{n} \cdot \vec{v}_1 \vec{S}_1 \times \vec{v}_1 \cdot \vec{v}_2 + \frac{45}{8} \hat{n} \cdot \vec{v}_2 \hat{n} \cdot \vec{v}_1 \hat{n} \times \vec{S}_1 \cdot \vec{v}_1 + \frac{9}{16} \vec{v}_1 \cdot \vec{v}_1 \hat{n} \times \vec{S}_1 \cdot \vec{v}_1 - \frac{9}{8} \vec{v}_1 \cdot \vec{v}_2 \hat{n} \times \vec{S}_1 \cdot \vec{v}_1 \Big) \Big) \Big\}$$

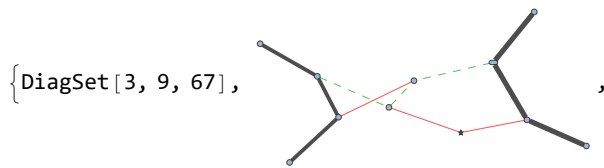

$$\frac{1}{r^3} G^3 m_1 m_2^2 \left( -2 \hat{n} \cdot \vec{a}_2 \hat{n} \times \vec{S}_1 \cdot \vec{v}_1 + \pi^2 \left( -\frac{9}{8} \hat{n} \cdot \vec{a}_2 \hat{n} \times \vec{S}_1 \cdot \vec{v}_1 - \frac{3}{4} \hat{n} \cdot \vec{v}_1 \hat{n} \times \vec{a}_2 \cdot \vec{S}_1 + \frac{5}{8} \vec{a}_2 \times \vec{S}_1 \cdot \vec{v}_1 + \frac{3}{4} \hat{n} \cdot \vec{v}_1 \hat{n} \times \vec{S}_1 \cdot \vec{v}_2 - \frac{9}{8} \hat{n} \cdot \vec{v}_2 \hat{n} \times \vec{S}_1 \cdot \vec{v}_1 + \frac{5}{8} \vec{S}_1 \times \vec{v}_1 \cdot \vec{v}_2 \right) - 2 \vec{a}_2 \times \vec{S}_1 \cdot \vec{v}_1 - 2 \hat{n} \cdot \vec{v}_2 \hat{n} \times \vec{S}_1 \cdot \vec{v}_1 - 2 \vec{S}_1 \times \vec{v}_1 \cdot \vec{v}_2 \right) + \frac{1}{r^4} G^3 m_1 m_2^2 \left( -10 (\hat{n} \cdot \vec{v}_2)^2 \hat{n} \times \vec{S}_1 \cdot \vec{v}_1 - 4 \hat{n} \cdot \vec{v}_2 \vec{S}_1 \times \vec{v}_1 \cdot \vec{v}_2 + 6 \hat{n} \cdot \vec{v}_1 \hat{n} \cdot \vec{v}_2 \hat{n} \times \vec{S}_1 \cdot \vec{v}_1 + 2 \hat{n} \cdot \vec{v}_1 \vec{S}_1 \times \vec{v}_1 \cdot \vec{v}_2 - 4 \vec{v}_1 \cdot \vec{v}_1 \hat{n} \times \vec{S}_1 \cdot \vec{v}_2 + 2 \vec{v}_1 \cdot \vec{v}_2 \hat{n} \times \vec{S}_1 \cdot \vec{v}_1 + 2 \vec{v}_2 \cdot \vec{v}_2 \hat{n} \times \vec{S}_1 \cdot \vec{v}_1 + \pi^2 \left( -\frac{45}{16} (\hat{n} \cdot \vec{v}_1)^2 \hat{n} \times \vec{S}_1 \cdot \vec{v}_2 - \frac{15}{8} \hat{n} \cdot \vec{v}_1 \vec{S}_1 \times \vec{v}_1 \cdot \vec{v}_2 + \frac{15}{4} \hat{n} \cdot \vec{v}_2 \hat{n} \cdot \vec{v}_1 \hat{n} \times \vec{S}_1 \cdot \vec{v}_1 + \frac{15}{4} \hat{n} \cdot \vec{v}_2 \hat{n} \cdot \vec{v}_1 \hat{n} \times \vec{S}_1 \cdot \vec{v}_2 - \frac{45}{8} (\hat{n} \cdot \vec{v}_2)^2 \hat{n} \times \vec{S}_1 \cdot \vec{v}_1 + 3 \hat{n} \cdot \vec{v}_2 \vec{S}_1 \times \vec{v}_1 \cdot \vec{v}_2 + \frac{9}{16} \vec{v}_1 \cdot \vec{v}_1 \hat{n} \times \vec{S}_1 \cdot \vec{v}_2 - \frac{3}{4} \vec{v}_1 \cdot \vec{v}_2 \hat{n} \times \vec{S}_1 \cdot \vec{v}_1 - \frac{3}{4} \vec{v}_1 \cdot \vec{v}_2 \hat{n} \times \vec{S}_1 \cdot \vec{v}_2 + \frac{9}{8} \vec{v}_2 \cdot \vec{v}_2 \hat{n} \times \vec{S}_1 \cdot \vec{v}_1 \right) \Big) \Big\}$$

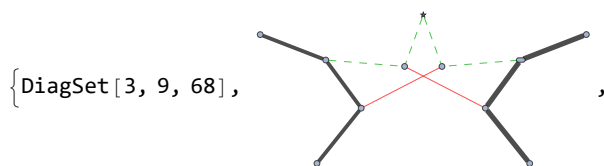

$$\frac{\left( \frac{3}{2} \pi^2 \hat{n} \times \vec{a}_2 \cdot \vec{S}_1 + 6 \hat{n} \times \vec{a}_2 \cdot \vec{S}_1 \right) m_1 m_2^2 G^3}{r^2} + \frac{1}{r^3} \left( 20 \vec{S}_1 \times \vec{v}_1 \cdot \vec{v}_2 - 14 \vec{a}_2 \times \vec{S}_1 \cdot \vec{v}_1 + 22 \vec{a}_2 \times \vec{S}_1 \cdot \vec{v}_2 + 30 \hat{n} \times \vec{S}_1 \cdot \vec{v}_1 \hat{n} \cdot \vec{a}_2 - 18 \hat{n} \times \vec{S}_1 \cdot \vec{v}_2 \hat{n} \cdot \vec{a}_2 + 22 \hat{n} \times \vec{S}_1 \cdot \vec{v}_2 \hat{n} \cdot \vec{v}_1 + 4 \hat{n} \times \vec{a}_2 \cdot \vec{S}_1 \hat{n} \cdot \vec{v}_1 - 30 \hat{n} \times \vec{S}_1 \cdot \vec{v}_1 \hat{n} \cdot \vec{v}_2 - 28 \hat{n} \times \vec{S}_1 \cdot \vec{v}_2 \hat{n} \cdot \vec{v}_2 - 28 \hat{n} \times \vec{a}_2 \cdot \vec{S}_1 \hat{n} \cdot \vec{v}_2 + \pi^2 \left( -\frac{3}{4} \vec{S}_1 \times \vec{v}_1 \cdot \vec{v}_2 + \frac{9}{4} \vec{a}_2 \times \vec{S}_1 \cdot \vec{v}_1 - \vec{a}_2 \times \vec{S}_1 \cdot \vec{v}_2 - \frac{9}{4} \hat{n} \times \vec{S}_1 \cdot \vec{v}_1 \hat{n} \cdot \vec{a}_2 - \frac{9}{2} \hat{n} \times \vec{a}_2 \cdot \vec{S}_1 \hat{n} \cdot \vec{v}_1 + \frac{9}{4} \hat{n} \times \vec{S}_1 \cdot \vec{v}_1 \hat{n} \cdot \vec{v}_2 - \frac{3}{2} \hat{n} \times \vec{S}_1 \cdot \vec{v}_2 \hat{n} \cdot \vec{v}_2 + 3 \hat{n} \times \vec{a}_2 \cdot \vec{S}_1 \hat{n} \cdot \vec{v}_2 \right) \right) m_1 m_2^2 G^3 + \frac{1}{r^4} \left( -\frac{59}{2} \hat{n} \times \vec{S}_1 \cdot \vec{v}_2 (\hat{n} \cdot \vec{v}_1)^2 - 22 \vec{S}_1 \times \vec{v}_1 \cdot \vec{v}_2 \hat{n} \cdot \vec{v}_1 + 35 \hat{n} \times \vec{S}_1 \cdot \vec{v}_1 \hat{n} \cdot \vec{v}_2 \hat{n} \cdot \vec{v}_1 + 212 \hat{n} \times \vec{S}_1 \cdot \vec{v}_2 \hat{n} \cdot \vec{v}_2 \hat{n} \cdot \vec{v}_1 - 95 \hat{n} \times \vec{S}_1 \cdot \vec{v}_1 (\hat{n} \cdot \vec{v}_2)^2 + \frac{21}{2} \hat{n} \times \vec{S}_1 \cdot \vec{v}_2 (\hat{n} \cdot \vec{v}_2)^2 + 82 \vec{S}_1 \times \vec{v}_1 \cdot \vec{v}_2 \hat{n} \cdot \vec{v}_2 + \frac{23}{2} \hat{n} \times \vec{S}_1 \cdot \vec{v}_2 \vec{v}_1 \cdot \vec{v}_1 - 7 \hat{n} \times \vec{S}_1 \cdot \vec{v}_1 \vec{v}_1 \cdot \vec{v}_2 - 36 \hat{n} \times \vec{S}_1 \cdot \vec{v}_2 \vec{v}_1 \cdot \vec{v}_2 + 19 \hat{n} \times \vec{S}_1 \cdot \vec{v}_1 \vec{v}_2 \cdot \vec{v}_2 - \frac{17}{2} \hat{n} \times \vec{S}_1 \cdot \vec{v}_2 \vec{v}_2 \cdot \vec{v}_2 + \pi^2 \left( -\frac{45}{32} \hat{n} \times \vec{S}_1 \cdot \vec{v}_2 (\hat{n} \cdot \vec{v}_1)^2 - \frac{45}{16} \hat{n} \times \vec{S}_1 \cdot \vec{v}_1 \hat{n} \cdot \vec{v}_2 \hat{n} \cdot \vec{v}_1 - \frac{45}{8} \hat{n} \times \vec{S}_1 \cdot \vec{v}_2 \hat{n} \cdot \vec{v}_2 \hat{n} \cdot \vec{v}_1 + \frac{165}{16} \hat{n} \times \vec{S}_1 \cdot \vec{v}_1 (\hat{n} \cdot \vec{v}_2)^2 - \frac{165}{32} \hat{n} \times \vec{S}_1 \cdot \vec{v}_2 (\hat{n} \cdot \vec{v}_2)^2 - \frac{21}{4} \vec{S}_1 \times \vec{v}_1 \cdot \vec{v}_2 \hat{n} \cdot \vec{v}_2 + \frac{9}{32} \hat{n} \times \vec{S}_1 \cdot \vec{v}_2 \vec{v}_1 \cdot \vec{v}_1 + \frac{9}{16} \hat{n} \times \vec{S}_1 \cdot \vec{v}_1 \vec{v}_1 \cdot \vec{v}_2 + \frac{9}{8} \hat{n} \times \vec{S}_1 \cdot \vec{v}_2 \vec{v}_1 \cdot \vec{v}_2 - \frac{33}{16} \hat{n} \times \vec{S}_1 \cdot \vec{v}_1 \vec{v}_2 \cdot \vec{v}_2 + \frac{33}{32} \hat{n} \times \vec{S}_1 \cdot \vec{v}_2 \vec{v}_2 \cdot \vec{v}_2 \right) \right) m_1 m_2^2 G^3 \Big\}$$

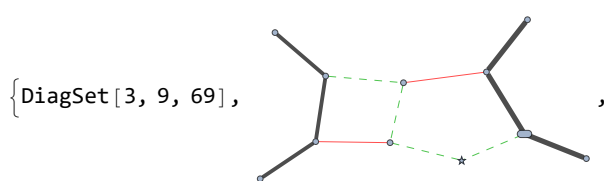

$$\begin{aligned}
& \frac{\left(2\pi^2 \hat{n} \times \vec{a}_2 \cdot \vec{S}_1 + 6\hat{n} \times \vec{a}_2 \cdot \vec{S}_1\right) m_1 m_2^2 G^3}{r^2} + \frac{1}{r^3} \left( -2\vec{S}_1 \times \vec{v}_1 \cdot \vec{v}_2 + 8\vec{a}_2 \times \vec{S}_1 \cdot \vec{v}_1 - 8\hat{n} \times \vec{S}_1 \cdot \vec{v}_1 \hat{n} \cdot \vec{a}_2 + 10\hat{n} \times \vec{S}_1 \cdot \vec{v}_2 \hat{n} \cdot \vec{v}_1 - \right. \\
& 8\hat{n} \times \vec{a}_2 \cdot \vec{S}_1 \hat{n} \cdot \vec{v}_1 + 8\hat{n} \times \vec{S}_1 \cdot \vec{v}_1 \hat{n} \cdot \vec{v}_2 - 18\hat{n} \times \vec{S}_1 \cdot \vec{v}_2 \hat{n} \cdot \vec{v}_2 + \pi^2 \left( \frac{9}{8} \vec{S}_1 \times \vec{v}_1 \cdot \vec{v}_2 + \frac{7}{8} \vec{a}_2 \times \vec{S}_1 \cdot \vec{v}_1 + \frac{9}{8} \hat{n} \times \vec{S}_1 \cdot \vec{v}_1 \hat{n} \cdot \vec{a}_2 + \right. \\
& \left. \frac{9}{4} \hat{n} \times \vec{S}_1 \cdot \vec{v}_2 \hat{n} \cdot \vec{v}_1 - \frac{15}{4} \hat{n} \times \vec{a}_2 \cdot \vec{S}_1 \hat{n} \cdot \vec{v}_1 - \frac{9}{8} \hat{n} \times \vec{S}_1 \cdot \vec{v}_1 \hat{n} \cdot \vec{v}_2 - 6\hat{n} \times \vec{S}_1 \cdot \vec{v}_2 \hat{n} \cdot \vec{v}_2 \right) \left. \right) m_1 m_2^2 G^3 + \frac{1}{r^4} \\
& \left( -\frac{33}{2} \hat{n} \times \vec{S}_1 \cdot \vec{v}_2 (\hat{n} \cdot \vec{v}_1)^2 - 12\vec{S}_1 \times \vec{v}_1 \cdot \vec{v}_2 \hat{n} \cdot \vec{v}_1 + 11\hat{n} \times \vec{S}_1 \cdot \vec{v}_1 \hat{n} \cdot \vec{v}_2 \hat{n} \cdot \vec{v}_1 + 40\hat{n} \times \vec{S}_1 \cdot \vec{v}_2 \hat{n} \cdot \vec{v}_2 \hat{n} \cdot \vec{v}_1 - \right. \\
& 40\hat{n} \times \vec{S}_1 \cdot \vec{v}_1 (\hat{n} \cdot \vec{v}_2)^2 + 32\vec{S}_1 \times \vec{v}_1 \cdot \vec{v}_2 \hat{n} \cdot \vec{v}_2 + \frac{5}{2} \hat{n} \times \vec{S}_1 \cdot \vec{v}_2 \vec{v}_1 \cdot \vec{v}_1 + \hat{n} \times \vec{S}_1 \cdot \vec{v}_1 \vec{v}_1 \cdot \vec{v}_2 - \\
& 8\hat{n} \times \vec{S}_1 \cdot \vec{v}_2 \vec{v}_1 \cdot \vec{v}_2 + 8\hat{n} \times \vec{S}_1 \cdot \vec{v}_1 \vec{v}_2 \cdot \vec{v}_2 + \pi^2 \left( -\frac{105}{32} \hat{n} \times \vec{S}_1 \cdot \vec{v}_2 (\hat{n} \cdot \vec{v}_1)^2 - \frac{9}{8} \vec{S}_1 \times \vec{v}_1 \cdot \vec{v}_2 \hat{n} \cdot \vec{v}_1 - \right. \\
& \frac{15}{16} \hat{n} \times \vec{S}_1 \cdot \vec{v}_1 \hat{n} \cdot \vec{v}_2 \hat{n} \cdot \vec{v}_1 + \frac{75}{4} \hat{n} \times \vec{S}_1 \cdot \vec{v}_2 \hat{n} \cdot \vec{v}_2 \hat{n} \cdot \vec{v}_1 + \frac{45}{8} \hat{n} \times \vec{S}_1 \cdot \vec{v}_1 (\hat{n} \cdot \vec{v}_2)^2 + \frac{3}{2} \vec{S}_1 \times \vec{v}_1 \cdot \vec{v}_2 \hat{n} \cdot \vec{v}_2 + \\
& \left. \frac{21}{32} \hat{n} \times \vec{S}_1 \cdot \vec{v}_2 \vec{v}_1 \cdot \vec{v}_1 + \frac{3}{16} \hat{n} \times \vec{S}_1 \cdot \vec{v}_1 \vec{v}_1 \cdot \vec{v}_2 - \frac{15}{4} \hat{n} \times \vec{S}_1 \cdot \vec{v}_2 \vec{v}_1 \cdot \vec{v}_2 - \frac{9}{8} \hat{n} \times \vec{S}_1 \cdot \vec{v}_1 \vec{v}_2 \cdot \vec{v}_2 \right) \left. \right) m_1 m_2^2 G^3 \Big\}
\end{aligned}$$

$\{\text{DiagSet}[3, 9, 70],$ 
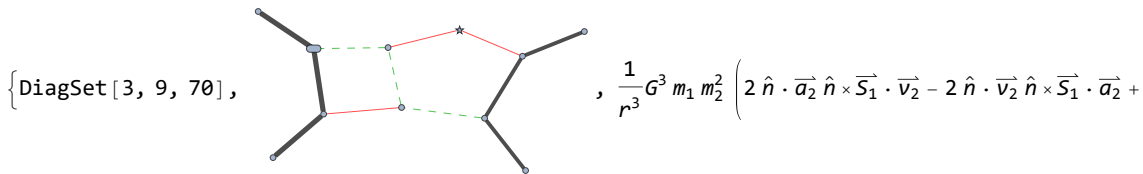
 $, \frac{1}{r^3} G^3 m_1 m_2^2 \left( 2\hat{n} \cdot \vec{a}_2 \hat{n} \times \vec{S}_1 \cdot \vec{v}_2 - 2\hat{n} \cdot \vec{v}_2 \hat{n} \times \vec{S}_1 \cdot \vec{a}_2 + \right.$

$$\begin{aligned}
& \pi^2 \left( -\frac{21}{8} \hat{n} \cdot \vec{a}_2 \hat{n} \times \vec{S}_1 \cdot \vec{v}_2 + \frac{9}{4} \hat{n} \cdot \vec{v}_2 \hat{n} \times \vec{S}_1 \cdot \vec{a}_2 + \frac{13}{8} \vec{S}_1 \times \vec{v}_2 \cdot \vec{a}_2 - \frac{3}{8} \hat{n} \cdot \vec{v}_2 \hat{n} \times \vec{S}_1 \cdot \vec{v}_2 \right) - 2\vec{S}_1 \times \vec{v}_2 \cdot \vec{a}_2 \Big) + \\
& \frac{1}{r^4} G^3 m_1 m_2^2 \left( -\frac{15}{2} (\hat{n} \cdot \vec{v}_2)^2 \hat{n} \times \vec{S}_1 \cdot \vec{v}_2 + \frac{3}{2} \vec{v}_2 \cdot \vec{v}_2 \hat{n} \times \vec{S}_1 \cdot \vec{v}_2 + \pi^2 \left( -\frac{15}{16} (\hat{n} \cdot \vec{v}_2)^2 \hat{n} \times \vec{S}_1 \cdot \vec{v}_2 + \right. \right. \\
& \left. \left. \frac{3}{8} \hat{n} \cdot \vec{v}_2 \vec{S}_1 \times \vec{v}_1 \cdot \vec{v}_2 + \frac{15}{8} \hat{n} \cdot \vec{v}_1 \hat{n} \cdot \vec{v}_2 \hat{n} \times \vec{S}_1 \cdot \vec{v}_2 - \frac{3}{8} \vec{v}_1 \cdot \vec{v}_2 \hat{n} \times \vec{S}_1 \cdot \vec{v}_2 + \frac{3}{16} \vec{v}_2 \cdot \vec{v}_2 \hat{n} \times \vec{S}_1 \cdot \vec{v}_2 \right) \right) \Big\}
\end{aligned}$$

$\{\text{DiagSet}[3, 9, 71],$ 
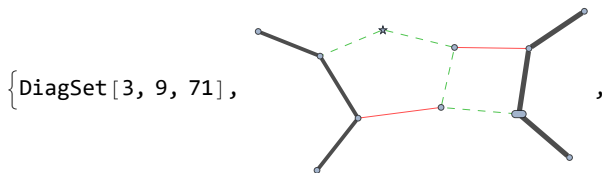
 $,$

$$\begin{aligned}
& \frac{1}{r^3} G^3 m_1 m_2^2 \left( 4\hat{n} \cdot \vec{a}_2 \hat{n} \times \vec{S}_1 \cdot \vec{v}_2 + 6\hat{n} \cdot \vec{v}_1 \hat{n} \times \vec{S}_1 \cdot \vec{a}_2 - 6\hat{n} \cdot \vec{v}_2 \hat{n} \times \vec{S}_1 \cdot \vec{a}_2 + \right. \\
& \pi^2 \left( -\frac{21}{8} \hat{n} \cdot \vec{a}_2 \hat{n} \times \vec{S}_1 \cdot \vec{v}_2 + \frac{3}{4} \hat{n} \cdot \vec{v}_1 \hat{n} \times \vec{S}_1 \cdot \vec{a}_2 + \frac{9}{4} \hat{n} \cdot \vec{v}_2 \hat{n} \times \vec{S}_1 \cdot \vec{a}_2 + \frac{1}{4} \vec{S}_1 \times \vec{v}_1 \cdot \vec{a}_2 + \right. \\
& \left. \frac{13}{8} \vec{S}_1 \times \vec{v}_2 \cdot \vec{a}_2 - \frac{3}{8} \hat{n} \cdot \vec{v}_2 \hat{n} \times \vec{S}_1 \cdot \vec{v}_2 \right) + 2\vec{S}_1 \times \vec{v}_1 \cdot \vec{a}_2 - 4\vec{S}_1 \times \vec{v}_2 \cdot \vec{a}_2 - 4\hat{n} \cdot \vec{v}_2 \hat{n} \times \vec{S}_1 \cdot \vec{v}_2 \Big) + \\
& \frac{G^3 m_1 m_2^2 \left( -\frac{1}{4} \pi^2 \hat{n} \times \vec{S}_1 \cdot \vec{a}_2 - 2\hat{n} \times \vec{S}_1 \cdot \vec{a}_2 \right)}{r^2} + \frac{1}{r^4} G^3 m_1 m_2^2 \left( -4(\hat{n} \cdot \vec{v}_2)^2 \hat{n} \times \vec{S}_1 \cdot \vec{v}_2 + 4\hat{n} \cdot \vec{v}_2 \vec{S}_1 \times \vec{v}_1 \cdot \vec{v}_2 + \right. \\
& 20\hat{n} \cdot \vec{v}_1 \hat{n} \cdot \vec{v}_2 \hat{n} \times \vec{S}_1 \cdot \vec{v}_2 - 4\vec{v}_1 \cdot \vec{v}_2 \hat{n} \times \vec{S}_1 \cdot \vec{v}_2 + \pi^2 \left( -\frac{15}{32} (\hat{n} \cdot \vec{v}_2)^2 \hat{n} \times \vec{S}_1 \cdot \vec{v}_2 + \right. \\
& \left. \frac{3}{8} \hat{n} \cdot \vec{v}_2 \vec{S}_1 \times \vec{v}_1 \cdot \vec{v}_2 + \frac{15}{8} \hat{n} \cdot \vec{v}_1 \hat{n} \cdot \vec{v}_2 \hat{n} \times \vec{S}_1 \cdot \vec{v}_2 - \frac{3}{8} \vec{v}_1 \cdot \vec{v}_2 \hat{n} \times \vec{S}_1 \cdot \vec{v}_2 + \frac{3}{32} \vec{v}_2 \cdot \vec{v}_2 \hat{n} \times \vec{S}_1 \cdot \vec{v}_2 \right) \Big\}
\end{aligned}$$

{DiagSet[3, 9, 72],

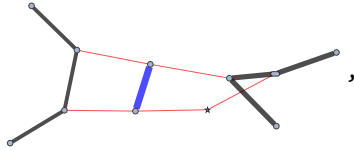

$$\begin{aligned} & \frac{1}{r^3} G^3 m_1 m_2^2 \left( -12 \hat{n} \cdot \vec{v}_1 \hat{n} \times \vec{a}_1 \cdot \vec{S}_1 + 18 \hat{n} \cdot \vec{v}_2 \hat{n} \times \vec{a}_1 \cdot \vec{S}_1 + \pi^2 \left( \frac{3}{4} \hat{n} \cdot \vec{v}_1 \hat{n} \times \vec{a}_1 \cdot \vec{S}_1 - \frac{3}{2} \hat{n} \cdot \vec{v}_2 \hat{n} \times \vec{a}_1 \cdot \vec{S}_1 - \right. \right. \\ & \quad \left. \frac{1}{4} \vec{a}_1 \times \vec{S}_1 \cdot \vec{v}_1 + \frac{1}{2} \vec{a}_1 \times \vec{S}_1 \cdot \vec{v}_2 - \frac{3}{4} \hat{n} \cdot \vec{v}_1 \hat{n} \times \vec{S}_1 \cdot \vec{v}_1 + \frac{3}{2} \hat{n} \cdot \vec{v}_2 \hat{n} \times \vec{S}_1 \cdot \vec{v}_1 - \frac{1}{2} \vec{S}_1 \times \vec{v}_1 \cdot \vec{v}_2 \right) + \\ & \quad \left. \frac{20}{3} \vec{a}_1 \times \vec{S}_1 \cdot \vec{v}_1 - 6 \vec{a}_1 \times \vec{S}_1 \cdot \vec{v}_2 + 12 \hat{n} \cdot \vec{v}_1 \hat{n} \times \vec{S}_1 \cdot \vec{v}_1 - 18 \hat{n} \cdot \vec{v}_2 \hat{n} \times \vec{S}_1 \cdot \vec{v}_1 + 6 \vec{S}_1 \times \vec{v}_1 \cdot \vec{v}_2 \right) + \frac{1}{r^4} \\ & G^3 m_1 m_2^2 \left( -\frac{34}{3} (\hat{n} \cdot \vec{v}_1)^2 \hat{n} \times \vec{S}_1 \cdot \vec{v}_1 - 6 \hat{n} \cdot \vec{v}_1 \vec{S}_1 \times \vec{v}_1 \cdot \vec{v}_2 + 30 \hat{n} \cdot \vec{v}_2 \hat{n} \times \vec{S}_1 \cdot \vec{v}_1 + \frac{14}{3} \vec{v}_1 \cdot \vec{v}_1 \hat{n} \times \vec{S}_1 \cdot \vec{v}_1 - \right. \\ & \quad \left. 6 \vec{v}_1 \cdot \vec{v}_2 \hat{n} \times \vec{S}_1 \cdot \vec{v}_1 + \pi^2 \left( \frac{15}{16} (\hat{n} \cdot \vec{v}_1)^2 \hat{n} \times \vec{S}_1 \cdot \vec{v}_1 + \frac{3}{4} \hat{n} \cdot \vec{v}_1 \vec{S}_1 \times \vec{v}_1 \cdot \vec{v}_2 - \right. \right. \\ & \quad \left. \left. \frac{15}{4} \hat{n} \cdot \vec{v}_2 \hat{n} \times \vec{S}_1 \cdot \vec{v}_1 - \frac{3}{16} \vec{v}_1 \cdot \vec{v}_1 \hat{n} \times \vec{S}_1 \cdot \vec{v}_1 + \frac{3}{4} \vec{v}_1 \cdot \vec{v}_2 \hat{n} \times \vec{S}_1 \cdot \vec{v}_1 \right) \right) \Bigg\} \end{aligned}$$

{DiagSet[3, 9, 73],

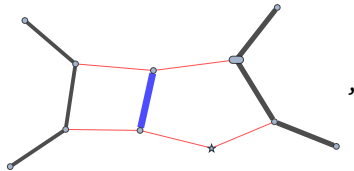

$$\begin{aligned} & \frac{1}{r^3} G^3 m_1 m_2^2 \left( -12 \hat{n} \cdot \vec{v}_1 \hat{n} \times \vec{a}_1 \cdot \vec{S}_1 + \pi^2 \left( \frac{3}{4} \hat{n} \cdot \vec{v}_1 \hat{n} \times \vec{a}_1 \cdot \vec{S}_1 - \frac{1}{4} \vec{a}_1 \times \vec{S}_1 \cdot \vec{v}_1 - \frac{3}{4} \hat{n} \cdot \vec{v}_1 \hat{n} \times \vec{S}_1 \cdot \vec{v}_1 \right) + \right. \\ & \quad \left. \frac{20}{3} \vec{a}_1 \times \vec{S}_1 \cdot \vec{v}_1 + 12 \hat{n} \cdot \vec{v}_1 \hat{n} \times \vec{S}_1 \cdot \vec{v}_1 \right) + \frac{1}{r^4} \\ & G^3 m_1 m_2^2 \left( -\frac{146}{3} (\hat{n} \cdot \vec{v}_1)^2 \hat{n} \times \vec{S}_1 \cdot \vec{v}_1 - 12 \hat{n} \cdot \vec{v}_1 \vec{S}_1 \times \vec{v}_1 \cdot \vec{v}_2 + 60 \hat{n} \cdot \vec{v}_2 \hat{n} \times \vec{S}_1 \cdot \vec{v}_1 + \frac{46}{3} \vec{v}_1 \cdot \vec{v}_1 \hat{n} \times \vec{S}_1 \cdot \vec{v}_1 - \right. \\ & \quad \left. 12 \vec{v}_1 \cdot \vec{v}_2 \hat{n} \times \vec{S}_1 \cdot \vec{v}_1 + \pi^2 \left( \frac{45}{16} (\hat{n} \cdot \vec{v}_1)^2 \hat{n} \times \vec{S}_1 \cdot \vec{v}_1 + \frac{3}{4} \hat{n} \cdot \vec{v}_1 \vec{S}_1 \times \vec{v}_1 \cdot \vec{v}_2 - \frac{15}{4} \hat{n} \cdot \vec{v}_2 \hat{n} \times \vec{S}_1 \cdot \vec{v}_1 - \right. \right. \\ & \quad \left. \left. \frac{9}{16} \vec{v}_1 \cdot \vec{v}_1 \hat{n} \times \vec{S}_1 \cdot \vec{v}_1 + \frac{3}{4} \vec{v}_1 \cdot \vec{v}_2 \hat{n} \times \vec{S}_1 \cdot \vec{v}_1 \right) \right) \Bigg\} \end{aligned}$$

{DiagSet[3, 9, 74],

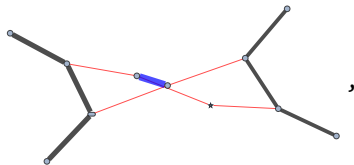

$$\begin{aligned} & \frac{1}{r^3} G^3 m_1 m_2^2 \left( -21 \hat{n} \cdot \vec{v}_2 \hat{n} \times \vec{S}_1 \cdot \vec{a}_1 + \pi^2 \left( \frac{3}{2} \hat{n} \cdot \vec{v}_2 \hat{n} \times \vec{S}_1 \cdot \vec{a}_1 - \frac{1}{2} \vec{S}_1 \times \vec{a}_1 \cdot \vec{v}_2 + \frac{3}{2} \hat{n} \cdot \vec{v}_2 \hat{n} \times \vec{S}_1 \cdot \vec{v}_1 - \frac{1}{2} \vec{S}_1 \times \vec{v}_1 \cdot \vec{v}_2 \right) + \right. \\ & \quad \left. \frac{25}{3} \vec{S}_1 \times \vec{a}_1 \cdot \vec{v}_2 - 21 \hat{n} \cdot \vec{v}_2 \hat{n} \times \vec{S}_1 \cdot \vec{v}_1 + \frac{25}{3} \vec{S}_1 \times \vec{v}_1 \cdot \vec{v}_2 \right) + \frac{1}{r^4} \\ & G^3 m_1 m_2^2 \left( -81 (\hat{n} \cdot \vec{v}_2)^2 \hat{n} \times \vec{S}_1 \cdot \vec{v}_1 + 34 \hat{n} \cdot \vec{v}_2 \vec{S}_1 \times \vec{v}_1 \cdot \vec{v}_2 + 105 \hat{n} \cdot \vec{v}_1 \hat{n} \cdot \vec{v}_2 \hat{n} \times \vec{S}_1 \cdot \vec{v}_1 - 25 \hat{n} \cdot \vec{v}_1 \vec{S}_1 \times \vec{v}_1 \cdot \vec{v}_2 - \right. \\ & \quad \left. 21 \vec{v}_1 \cdot \vec{v}_2 \hat{n} \times \vec{S}_1 \cdot \vec{v}_1 + 21 \vec{v}_2 \cdot \vec{v}_2 \hat{n} \times \vec{S}_1 \cdot \vec{v}_1 + \pi^2 \left( \frac{45}{8} (\hat{n} \cdot \vec{v}_2)^2 \hat{n} \times \vec{S}_1 \cdot \vec{v}_1 - \frac{9}{4} \hat{n} \cdot \vec{v}_2 \vec{S}_1 \times \vec{v}_1 \cdot \vec{v}_2 - \right. \right. \\ & \quad \left. \left. \frac{15}{2} \hat{n} \cdot \vec{v}_1 \hat{n} \cdot \vec{v}_2 \hat{n} \times \vec{S}_1 \cdot \vec{v}_1 + \frac{3}{2} \hat{n} \cdot \vec{v}_1 \vec{S}_1 \times \vec{v}_1 \cdot \vec{v}_2 + \frac{3}{2} \vec{v}_1 \cdot \vec{v}_2 \hat{n} \times \vec{S}_1 \cdot \vec{v}_1 - \frac{9}{8} \vec{v}_2 \cdot \vec{v}_2 \hat{n} \times \vec{S}_1 \cdot \vec{v}_1 \right) \right) \Bigg\} \end{aligned}$$

{DiagSet[3, 9, 75],

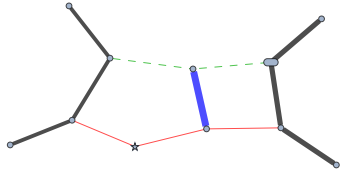

,

$$\frac{1}{r^3} G^3 m_1 m_2^2 \left( -\hat{n} \cdot \vec{a}_2 \hat{n} \times \vec{S}_1 \cdot \vec{v}_2 + 20 \hat{n} \cdot \vec{v}_2 \hat{n} \times \vec{S}_1 \cdot \vec{a}_2 + \pi^2 \left( -\frac{3}{2} \hat{n} \cdot \vec{v}_2 \hat{n} \times \vec{S}_1 \cdot \vec{a}_2 - \frac{1}{2} \vec{S}_1 \times \vec{v}_2 \cdot \vec{a}_2 - \frac{3}{2} \hat{n} \cdot \vec{v}_2 \hat{n} \times \vec{S}_1 \cdot \vec{v}_2 \right) + \right. \\ \left. \frac{25}{3} \vec{S}_1 \times \vec{v}_2 \cdot \vec{a}_2 + 19 \hat{n} \cdot \vec{v}_2 \hat{n} \times \vec{S}_1 \cdot \vec{v}_2 \right) + \frac{1}{r^4} \\ G^3 m_1 m_2^2 \left( \frac{127}{2} (\hat{n} \cdot \vec{v}_2)^2 \hat{n} \times \vec{S}_1 \cdot \vec{v}_2 - 19 \hat{n} \cdot \vec{v}_2 \vec{S}_1 \times \vec{v}_1 \cdot \vec{v}_2 - 95 \hat{n} \cdot \vec{v}_1 \hat{n} \cdot \vec{v}_2 \hat{n} \times \vec{S}_1 \cdot \vec{v}_2 + 19 \vec{v}_1 \cdot \vec{v}_2 \hat{n} \times \vec{S}_1 \cdot \vec{v}_2 - \right. \\ \left. \frac{43}{2} \vec{v}_2 \cdot \vec{v}_2 \hat{n} \times \vec{S}_1 \cdot \vec{v}_2 + \pi^2 \left( -\frac{135}{32} (\hat{n} \cdot \vec{v}_2)^2 \hat{n} \times \vec{S}_1 \cdot \vec{v}_2 + \frac{3}{2} \hat{n} \cdot \vec{v}_2 \vec{S}_1 \times \vec{v}_1 \cdot \vec{v}_2 + \right. \right. \\ \left. \left. \frac{15}{2} \hat{n} \cdot \vec{v}_1 \hat{n} \cdot \vec{v}_2 \hat{n} \times \vec{S}_1 \cdot \vec{v}_2 - \frac{3}{2} \vec{v}_1 \cdot \vec{v}_2 \hat{n} \times \vec{S}_1 \cdot \vec{v}_2 + \frac{27}{32} \vec{v}_2 \cdot \vec{v}_2 \hat{n} \times \vec{S}_1 \cdot \vec{v}_2 \right) \right) \Bigg\}$$

{DiagSet[3, 9, 76],

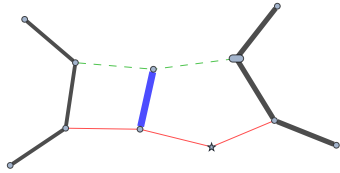

,  $\frac{1}{r^3} G^3 m_1 m_2^2$

$$\left( 4 \hat{n} \cdot \vec{a}_2 \hat{n} \times \vec{S}_1 \cdot \vec{v}_1 + 11 \hat{n} \cdot \vec{v}_1 \hat{n} \times \vec{a}_2 \cdot \vec{S}_1 + \pi^2 \left( -\frac{3}{4} \hat{n} \cdot \vec{v}_1 \hat{n} \times \vec{a}_2 \cdot \vec{S}_1 + \frac{1}{4} \vec{a}_2 \times \vec{S}_1 \cdot \vec{v}_1 + \frac{3}{4} \hat{n} \cdot \vec{v}_1 \hat{n} \times \vec{S}_1 \cdot \vec{v}_2 + \frac{1}{4} \vec{S}_1 \times \vec{v}_1 \cdot \vec{v}_2 \right) - \right. \\ \left. \frac{23}{3} \vec{a}_2 \times \vec{S}_1 \cdot \vec{v}_1 - 11 \hat{n} \cdot \vec{v}_1 \hat{n} \times \vec{S}_1 \cdot \vec{v}_2 + 4 \hat{n} \cdot \vec{v}_2 \hat{n} \times \vec{S}_1 \cdot \vec{v}_1 - \frac{23}{3} \vec{S}_1 \times \vec{v}_1 \cdot \vec{v}_2 \right) + \frac{1}{r^4} \\ G^3 m_1 m_2^2 \left( \frac{511}{12} (\hat{n} \cdot \vec{v}_1)^2 \hat{n} \times \vec{S}_1 \cdot \vec{v}_2 + \frac{62}{3} \hat{n} \cdot \vec{v}_1 \vec{S}_1 \times \vec{v}_1 \cdot \vec{v}_2 - \frac{13}{6} \hat{n} \cdot \vec{v}_2 \hat{n} \cdot \vec{v}_1 \hat{n} \times \vec{S}_1 \cdot \vec{v}_1 - 55 \hat{n} \cdot \vec{v}_2 \hat{n} \cdot \vec{v}_1 \hat{n} \times \vec{S}_1 \cdot \vec{v}_2 + \right. \\ \left. 20 (\hat{n} \cdot \vec{v}_2)^2 \hat{n} \times \vec{S}_1 \cdot \vec{v}_1 - 27 \hat{n} \cdot \vec{v}_2 \vec{S}_1 \times \vec{v}_1 \cdot \vec{v}_2 - \frac{179}{12} \vec{v}_1 \cdot \vec{v}_1 \hat{n} \times \vec{S}_1 \cdot \vec{v}_2 - \frac{7}{6} \vec{v}_1 \cdot \vec{v}_2 \hat{n} \times \vec{S}_1 \cdot \vec{v}_1 + 11 \vec{v}_1 \cdot \vec{v}_2 \hat{n} \times \vec{S}_1 \cdot \vec{v}_2 + \right. \\ \left. \pi^2 \left( -\frac{165}{64} (\hat{n} \cdot \vec{v}_1)^2 \hat{n} \times \vec{S}_1 \cdot \vec{v}_2 - \frac{3}{4} \hat{n} \cdot \vec{v}_1 \vec{S}_1 \times \vec{v}_1 \cdot \vec{v}_2 - \frac{45}{32} \hat{n} \cdot \vec{v}_2 \hat{n} \cdot \vec{v}_1 \hat{n} \times \vec{S}_1 \cdot \vec{v}_1 + \frac{15}{4} \hat{n} \cdot \vec{v}_2 \hat{n} \cdot \vec{v}_1 \hat{n} \times \vec{S}_1 \cdot \vec{v}_2 + \right. \right. \\ \left. \left. \frac{3}{4} \hat{n} \cdot \vec{v}_2 \vec{S}_1 \times \vec{v}_1 \cdot \vec{v}_2 + \frac{33}{64} \vec{v}_1 \cdot \vec{v}_1 \hat{n} \times \vec{S}_1 \cdot \vec{v}_2 + \frac{9}{32} \vec{v}_1 \cdot \vec{v}_2 \hat{n} \times \vec{S}_1 \cdot \vec{v}_1 - \frac{3}{4} \vec{v}_1 \cdot \vec{v}_2 \hat{n} \times \vec{S}_1 \cdot \vec{v}_2 \right) - 4 \vec{v}_2 \cdot \vec{v}_2 \hat{n} \times \vec{S}_1 \cdot \vec{v}_1 \right) \Bigg\}$$

{DiagSet[3, 9, 77],

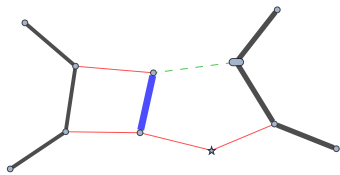

,

$$\frac{\left( 5 \hat{n} \times \vec{S}_1 \cdot \vec{v}_1 - \frac{1}{4} \pi^2 \hat{n} \times \vec{S}_1 \cdot \vec{v}_1 \right) m_1 m_2^2 G^3}{r^2} + \frac{1}{r^3} \left( -\frac{21}{2} \vec{S}_1 \times \vec{v}_1 \cdot \vec{v}_2 + 5 \vec{a}_1 \times \vec{S}_1 \cdot \vec{v}_1 - \frac{11}{2} \vec{a}_2 \times \vec{S}_1 \cdot \vec{v}_1 - \frac{40}{3} \hat{n} \times \vec{S}_1 \cdot \vec{v}_1 \hat{n} \cdot \vec{a}_1 + \right. \\ \left. \frac{44}{3} \hat{n} \times \vec{S}_1 \cdot \vec{v}_1 \hat{n} \cdot \vec{a}_2 - \frac{70}{3} \hat{n} \times \vec{S}_1 \cdot \vec{v}_1 \hat{n} \cdot \vec{v}_1 - \frac{23}{6} \hat{n} \times \vec{S}_1 \cdot \vec{v}_2 \hat{n} \cdot \vec{v}_1 - \frac{5}{3} \hat{n} \times \vec{a}_1 \cdot \vec{S}_1 \hat{n} \cdot \vec{v}_1 + \frac{23}{6} \hat{n} \times \vec{a}_2 \cdot \vec{S}_1 \hat{n} \cdot \vec{v}_1 + \right. \\ \left. \frac{89}{3} \hat{n} \times \vec{S}_1 \cdot \vec{v}_1 \hat{n} \cdot \vec{v}_2 + \pi^2 \left( \frac{3}{4} \vec{S}_1 \times \vec{v}_1 \cdot \vec{v}_2 - \frac{1}{4} \vec{a}_1 \times \vec{S}_1 \cdot \vec{v}_1 + \frac{1}{2} \vec{a}_2 \times \vec{S}_1 \cdot \vec{v}_1 + \frac{3}{4} \hat{n} \times \vec{S}_1 \cdot \vec{v}_1 \hat{n} \cdot \vec{a}_1 - \frac{9}{8} \hat{n} \times \vec{S}_1 \cdot \vec{v}_1 \hat{n} \cdot \vec{a}_2 + \right. \right. \\ \left. \left. \frac{3}{2} \hat{n} \times \vec{S}_1 \cdot \vec{v}_1 \hat{n} \cdot \vec{v}_1 + \frac{3}{8} \hat{n} \times \vec{S}_1 \cdot \vec{v}_2 \hat{n} \cdot \vec{v}_1 - \frac{3}{8} \hat{n} \times \vec{a}_2 \cdot \vec{S}_1 \hat{n} \cdot \vec{v}_1 - \frac{15}{8} \hat{n} \times \vec{S}_1 \cdot \vec{v}_1 \hat{n} \cdot \vec{v}_2 \right) \right) m_1 m_2^2 G^3 + \frac{1}{r^4} \\ \left( \frac{593}{12} \hat{n} \times \vec{S}_1 \cdot \vec{v}_1 (\hat{n} \cdot \vec{v}_1)^2 + \frac{421}{24} \hat{n} \times \vec{S}_1 \cdot \vec{v}_2 (\hat{n} \cdot \vec{v}_1)^2 + \frac{98}{3} \vec{S}_1 \times \vec{v}_1 \cdot \vec{v}_2 \hat{n} \cdot \vec{v}_1 - \frac{529}{4} \hat{n} \times \vec{S}_1 \cdot \vec{v}_1 \hat{n} \cdot \vec{v}_2 \hat{n} \cdot \vec{v}_1 - \right.$$

$$\begin{aligned} & \frac{115}{6} \hat{n} \times \vec{S}_1 \cdot \vec{v}_2 \hat{n} \cdot \vec{v}_2 \hat{n} \cdot \vec{v}_1 + \frac{220}{3} \hat{n} \times \vec{S}_1 \cdot \vec{v}_1 (\hat{n} \cdot \vec{v}_2)^2 - \frac{187}{6} \vec{S}_1 \times \vec{v}_1 \cdot \vec{v}_2 \hat{n} \cdot \vec{v}_2 - \frac{205}{12} \hat{n} \times \vec{S}_1 \cdot \vec{v}_1 \vec{v}_1 \cdot \vec{v}_1 - \\ & \frac{17}{24} \hat{n} \times \vec{S}_1 \cdot \vec{v}_2 \vec{v}_1 \cdot \vec{v}_1 + \frac{117}{4} \hat{n} \times \vec{S}_1 \cdot \vec{v}_1 \vec{v}_1 \cdot \vec{v}_2 + \frac{23}{6} \hat{n} \times \vec{S}_1 \cdot \vec{v}_2 \vec{v}_1 \cdot \vec{v}_2 - \frac{44}{3} \hat{n} \times \vec{S}_1 \cdot \vec{v}_1 \vec{v}_2 \cdot \vec{v}_2 + \\ & \pi^2 \left( -\frac{195}{64} \hat{n} \times \vec{S}_1 \cdot \vec{v}_1 (\hat{n} \cdot \vec{v}_1)^2 - \frac{255}{128} \hat{n} \times \vec{S}_1 \cdot \vec{v}_2 (\hat{n} \cdot \vec{v}_1)^2 - \frac{45}{16} \vec{S}_1 \times \vec{v}_1 \cdot \vec{v}_2 \hat{n} \cdot \vec{v}_1 + \frac{645}{64} \hat{n} \times \vec{S}_1 \cdot \vec{v}_1 \hat{n} \cdot \vec{v}_2 \hat{n} \cdot \vec{v}_1 + \right. \\ & \frac{15}{8} \hat{n} \times \vec{S}_1 \cdot \vec{v}_2 \hat{n} \cdot \vec{v}_2 \hat{n} \cdot \vec{v}_1 - \frac{45}{8} \hat{n} \times \vec{S}_1 \cdot \vec{v}_1 (\hat{n} \cdot \vec{v}_2)^2 + \frac{21}{8} \vec{S}_1 \times \vec{v}_1 \cdot \vec{v}_2 \hat{n} \cdot \vec{v}_2 + \frac{39}{64} \hat{n} \times \vec{S}_1 \cdot \vec{v}_1 \vec{v}_1 \cdot \vec{v}_1 + \\ & \left. \frac{51}{128} \hat{n} \times \vec{S}_1 \cdot \vec{v}_2 \vec{v}_1 \cdot \vec{v}_1 - \frac{129}{64} \hat{n} \times \vec{S}_1 \cdot \vec{v}_1 \vec{v}_1 \cdot \vec{v}_2 - \frac{3}{8} \hat{n} \times \vec{S}_1 \cdot \vec{v}_2 \vec{v}_1 \cdot \vec{v}_2 + \frac{9}{8} \hat{n} \times \vec{S}_1 \cdot \vec{v}_1 \vec{v}_2 \cdot \vec{v}_2 \right) \left. \right\} m_1 m_2^2 G^3 \end{aligned}$$

{DiagSet[3, 9, 78],

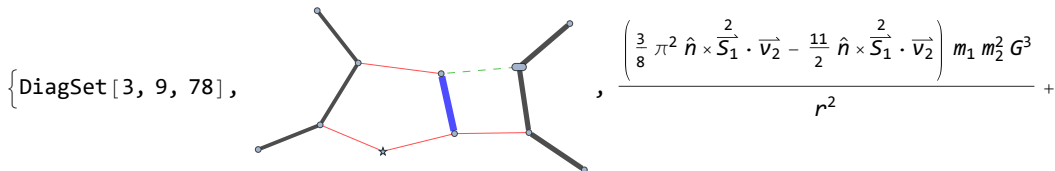

,  $\frac{\left( \frac{3}{8} \pi^2 \hat{n} \times \vec{S}_1 \cdot \vec{v}_2 - \frac{11}{2} \hat{n} \times \vec{S}_1 \cdot \vec{v}_2 \right) m_1 m_2^2 G^3}{r^2} +$

$$\begin{aligned} & \frac{1}{r^3} \left( 7 \frac{1}{\vec{S}_1 \times \vec{v}_1 \cdot \vec{v}_2} + \frac{3}{2} \vec{S}_1 \times \vec{a}_1 \cdot \vec{v}_2 + \frac{3}{2} \vec{S}_1 \times \vec{v}_2 \cdot \vec{a}_2 + \frac{26}{3} \hat{n} \times \vec{S}_1 \cdot \vec{v}_2 \hat{n} \cdot \vec{a}_1 - \frac{31}{3} \hat{n} \times \vec{S}_1 \cdot \vec{v}_2 \hat{n} \cdot \vec{a}_2 + \right. \\ & \frac{151}{6} \hat{n} \times \vec{S}_1 \cdot \vec{v}_2 \hat{n} \cdot \vec{v}_1 + \frac{25}{6} \hat{n} \times \vec{S}_1 \cdot \vec{v}_1 \hat{n} \cdot \vec{v}_2 - \frac{91}{3} \hat{n} \times \vec{S}_1 \cdot \vec{v}_2 \hat{n} \cdot \vec{v}_2 + \frac{25}{6} \hat{n} \times \vec{S}_1 \cdot \vec{a}_1 \hat{n} \cdot \vec{v}_2 - \frac{35}{6} \hat{n} \times \vec{S}_1 \cdot \vec{a}_2 \hat{n} \cdot \vec{v}_2 + \\ & \pi^2 \left( -\frac{5}{16} \frac{1}{\vec{S}_1 \times \vec{v}_1 \cdot \vec{v}_2} + \frac{1}{16} \vec{S}_1 \times \vec{a}_1 \cdot \vec{v}_2 + \frac{1}{8} \vec{S}_1 \times \vec{v}_2 \cdot \vec{a}_2 - \frac{3}{8} \hat{n} \times \vec{S}_1 \cdot \vec{v}_2 \hat{n} \cdot \vec{a}_1 + \frac{3}{8} \hat{n} \times \vec{S}_1 \cdot \vec{v}_2 \hat{n} \cdot \vec{a}_2 - \frac{3}{2} \hat{n} \times \vec{S}_1 \cdot \vec{v}_2 \hat{n} \cdot \vec{v}_1 - \right. \\ & \frac{9}{16} \hat{n} \times \vec{S}_1 \cdot \vec{v}_1 \hat{n} \cdot \vec{v}_2 + \frac{9}{4} \hat{n} \times \vec{S}_1 \cdot \vec{v}_2 \hat{n} \cdot \vec{v}_2 - \frac{9}{16} \hat{n} \times \vec{S}_1 \cdot \vec{a}_1 \hat{n} \cdot \vec{v}_2 + \frac{3}{4} \hat{n} \times \vec{S}_1 \cdot \vec{a}_2 \hat{n} \cdot \vec{v}_2 \left. \right) \left. \right\} m_1 m_2^2 G^3 + \frac{1}{r^4} \\ & \left( -\frac{130}{3} \hat{n} \times \vec{S}_1 \cdot \vec{v}_2 (\hat{n} \cdot \vec{v}_1)^2 - \frac{79}{6} \vec{S}_1 \times \vec{v}_1 \cdot \vec{v}_2 \hat{n} \cdot \vec{v}_1 - \frac{125}{6} \hat{n} \times \vec{S}_1 \cdot \vec{v}_1 \hat{n} \cdot \vec{v}_2 \hat{n} \cdot \vec{v}_1 + 150 \hat{n} \times \vec{S}_1 \cdot \vec{v}_2 \hat{n} \cdot \vec{v}_2 \hat{n} \cdot \vec{v}_1 + \right. \\ & \frac{31}{12} \hat{n} \times \vec{S}_1 \cdot \vec{v}_1 (\hat{n} \cdot \vec{v}_2)^2 - \frac{1735}{24} \hat{n} \times \vec{S}_1 \cdot \vec{v}_2 (\hat{n} \cdot \vec{v}_2)^2 + \frac{175}{6} \vec{S}_1 \times \vec{v}_1 \cdot \vec{v}_2 \hat{n} \cdot \vec{v}_2 + \frac{26}{3} \hat{n} \times \vec{S}_1 \cdot \vec{v}_2 \vec{v}_1 \cdot \vec{v}_1 + \\ & \frac{25}{6} \hat{n} \times \vec{S}_1 \cdot \vec{v}_1 \vec{v}_1 \cdot \vec{v}_2 - 32 \hat{n} \times \vec{S}_1 \cdot \vec{v}_2 \vec{v}_1 \cdot \vec{v}_2 - \frac{47}{12} \hat{n} \times \vec{S}_1 \cdot \vec{v}_1 \vec{v}_2 \cdot \vec{v}_2 + \frac{491}{24} \hat{n} \times \vec{S}_1 \cdot \vec{v}_2 \vec{v}_2 \cdot \vec{v}_2 + \\ & \pi^2 \left( \frac{15}{8} \hat{n} \times \vec{S}_1 \cdot \vec{v}_2 (\hat{n} \cdot \vec{v}_1)^2 + \frac{3}{16} \vec{S}_1 \times \vec{v}_1 \cdot \vec{v}_2 \hat{n} \cdot \vec{v}_1 + \frac{45}{16} \hat{n} \times \vec{S}_1 \cdot \vec{v}_1 \hat{n} \cdot \vec{v}_2 \hat{n} \cdot \vec{v}_1 - \frac{345}{32} \hat{n} \times \vec{S}_1 \cdot \vec{v}_2 \hat{n} \cdot \vec{v}_2 \hat{n} \cdot \vec{v}_1 - \right. \\ & \frac{15}{64} \hat{n} \times \vec{S}_1 \cdot \vec{v}_1 (\hat{n} \cdot \vec{v}_2)^2 + \frac{645}{128} \hat{n} \times \vec{S}_1 \cdot \vec{v}_2 (\hat{n} \cdot \vec{v}_2)^2 - \frac{33}{16} \vec{S}_1 \times \vec{v}_1 \cdot \vec{v}_2 \hat{n} \cdot \vec{v}_2 - \frac{3}{8} \hat{n} \times \vec{S}_1 \cdot \vec{v}_2 \vec{v}_1 \cdot \vec{v}_1 - \\ & \left. \frac{9}{16} \hat{n} \times \vec{S}_1 \cdot \vec{v}_1 \vec{v}_1 \cdot \vec{v}_2 + \frac{69}{32} \hat{n} \times \vec{S}_1 \cdot \vec{v}_2 \vec{v}_1 \cdot \vec{v}_2 + \frac{3}{64} \hat{n} \times \vec{S}_1 \cdot \vec{v}_1 \vec{v}_2 \cdot \vec{v}_2 - \frac{129}{128} \hat{n} \times \vec{S}_1 \cdot \vec{v}_2 \vec{v}_2 \cdot \vec{v}_2 \right) \left. \right\} m_1 m_2^2 G^3 \end{aligned}$$

{DiagSet[3, 9, 79],

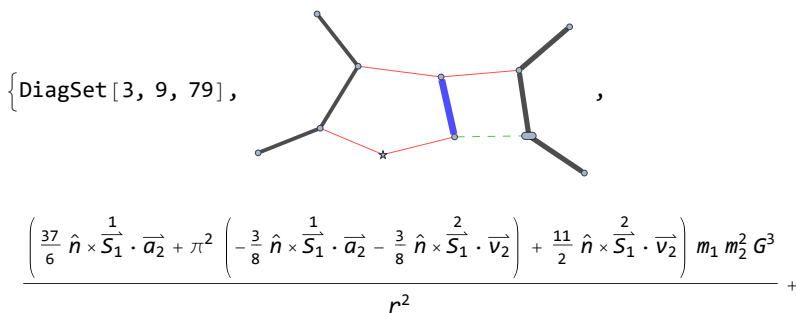

,  $\frac{\left( \frac{37}{6} \hat{n} \times \vec{S}_1 \cdot \vec{a}_2 + \pi^2 \left( -\frac{3}{8} \hat{n} \times \vec{S}_1 \cdot \vec{a}_2 - \frac{3}{8} \hat{n} \times \vec{S}_1 \cdot \vec{v}_2 \right) + \frac{11}{2} \hat{n} \times \vec{S}_1 \cdot \vec{v}_2 \right) m_1 m_2^2 G^3}{r^2} +$

$$\begin{aligned} & \frac{1}{r^3} \left( -\frac{17}{2} \frac{1}{\vec{S}_1 \times \vec{v}_1 \cdot \vec{v}_2} - 3 \vec{S}_1 \times \vec{a}_1 \cdot \vec{v}_2 - \frac{37}{6} \vec{S}_1 \times \vec{v}_1 \cdot \vec{a}_2 + \frac{37}{6} \vec{S}_1 \times \vec{v}_2 \cdot \vec{a}_2 - \right. \\ & \frac{19}{3} \hat{n} \times \vec{S}_1 \cdot \vec{v}_2 \hat{n} \cdot \vec{a}_1 - \frac{11}{6} \hat{n} \times \vec{S}_1 \cdot \vec{v}_2 \hat{n} \cdot \vec{a}_2 - \frac{137}{6} \hat{n} \times \vec{S}_1 \cdot \vec{v}_2 \hat{n} \cdot \vec{v}_1 - \frac{37}{2} \hat{n} \times \vec{S}_1 \cdot \vec{a}_2 \hat{n} \cdot \vec{v}_1 + \\ & \frac{8}{3} \hat{n} \times \vec{S}_1 \cdot \vec{v}_1 \hat{n} \cdot \vec{v}_2 + \frac{107}{6} \hat{n} \times \vec{S}_1 \cdot \vec{v}_2 \hat{n} \cdot \vec{v}_2 + \frac{8}{3} \hat{n} \times \vec{S}_1 \cdot \vec{a}_1 \hat{n} \cdot \vec{v}_2 + \frac{50}{3} \hat{n} \times \vec{S}_1 \cdot \vec{a}_2 \hat{n} \cdot \vec{v}_2 + \end{aligned}$$

$$\begin{aligned}
& \pi^2 \left( \frac{9}{16} \vec{S}_1 \times \vec{v}_1 \cdot \vec{v}_2 + \frac{3}{16} \vec{S}_1 \times \vec{a}_1 \cdot \vec{v}_2 + \frac{3}{8} \vec{S}_1 \times \vec{v}_1 \cdot \vec{a}_2 - \frac{3}{8} \vec{S}_1 \times \vec{v}_2 \cdot \vec{a}_2 + \frac{3}{8} \hat{n} \times \vec{S}_1 \cdot \vec{v}_2 \hat{n} \cdot \vec{a}_1 + \frac{3}{2} \hat{n} \times \vec{S}_1 \cdot \vec{v}_2 \hat{n} \cdot \vec{v}_1 + \right. \\
& \quad \left. \frac{9}{8} \hat{n} \times \vec{S}_1 \cdot \vec{a}_2 \hat{n} \cdot \vec{v}_1 - \frac{3}{16} \hat{n} \times \vec{S}_1 \cdot \vec{v}_1 \hat{n} \cdot \vec{v}_2 - \frac{9}{8} \hat{n} \times \vec{S}_1 \cdot \vec{v}_2 \hat{n} \cdot \vec{v}_2 - \frac{3}{16} \hat{n} \times \vec{S}_1 \cdot \vec{a}_1 \hat{n} \cdot \vec{v}_2 - \frac{9}{8} \hat{n} \times \vec{S}_1 \cdot \vec{a}_2 \hat{n} \cdot \vec{v}_2 \right) \\
& m_1 m_2^2 G^3 + \frac{1}{r^4} \left( \frac{95}{3} \hat{n} \times \vec{S}_1 \cdot \vec{v}_2 (\hat{n} \cdot \vec{v}_1)^2 + \frac{46}{3} \vec{S}_1 \times \vec{v}_1 \cdot \vec{v}_2 \hat{n} \cdot \vec{v}_1 - \frac{40}{3} \hat{n} \times \vec{S}_1 \cdot \vec{v}_1 \hat{n} \cdot \vec{v}_2 \hat{n} \cdot \vec{v}_1 - \right. \\
& \quad \frac{15}{2} \hat{n} \times \vec{S}_1 \cdot \vec{v}_2 \hat{n} \cdot \vec{v}_2 \hat{n} \cdot \vec{v}_1 - \frac{119}{12} \hat{n} \times \vec{S}_1 \cdot \vec{v}_1 (\hat{n} \cdot \vec{v}_2)^2 + \frac{305}{24} \hat{n} \times \vec{S}_1 \cdot \vec{v}_2 (\hat{n} \cdot \vec{v}_2)^2 + \frac{8}{3} \vec{S}_1 \times \vec{v}_1 \cdot \vec{v}_2 \hat{n} \cdot \vec{v}_2 - \\
& \quad \frac{19}{3} \hat{n} \times \vec{S}_1 \cdot \vec{v}_2 \vec{v}_1 \cdot \vec{v}_1 + \frac{8}{3} \hat{n} \times \vec{S}_1 \cdot \vec{v}_1 \vec{v}_1 \cdot \vec{v}_2 - \frac{1}{2} \hat{n} \times \vec{S}_1 \cdot \vec{v}_2 \vec{v}_1 \cdot \vec{v}_2 - \frac{17}{12} \hat{n} \times \vec{S}_1 \cdot \vec{v}_1 \vec{v}_2 \cdot \vec{v}_2 + \frac{83}{24} \hat{n} \times \vec{S}_1 \cdot \vec{v}_2 \vec{v}_2 \cdot \vec{v}_2 + \\
& \quad \pi^2 \left( -\frac{15}{8} \hat{n} \times \vec{S}_1 \cdot \vec{v}_2 (\hat{n} \cdot \vec{v}_1)^2 - \frac{15}{16} \vec{S}_1 \times \vec{v}_1 \cdot \vec{v}_2 \hat{n} \cdot \vec{v}_1 + \frac{15}{16} \hat{n} \times \vec{S}_1 \cdot \vec{v}_1 \hat{n} \cdot \vec{v}_2 \hat{n} \cdot \vec{v}_1 - \frac{45}{32} \hat{n} \times \vec{S}_1 \cdot \vec{v}_2 \hat{n} \cdot \vec{v}_2 \hat{n} \cdot \vec{v}_1 + \right. \\
& \quad \frac{105}{64} \hat{n} \times \vec{S}_1 \cdot \vec{v}_1 (\hat{n} \cdot \vec{v}_2)^2 - \frac{135}{128} \hat{n} \times \vec{S}_1 \cdot \vec{v}_2 (\hat{n} \cdot \vec{v}_2)^2 - \frac{15}{16} \vec{S}_1 \times \vec{v}_1 \cdot \vec{v}_2 \hat{n} \cdot \vec{v}_2 + \frac{3}{8} \hat{n} \times \vec{S}_1 \cdot \vec{v}_2 \vec{v}_1 \cdot \vec{v}_1 - \\
& \quad \left. \frac{3}{16} \hat{n} \times \vec{S}_1 \cdot \vec{v}_1 \vec{v}_1 \cdot \vec{v}_2 + \frac{9}{32} \hat{n} \times \vec{S}_1 \cdot \vec{v}_2 \vec{v}_1 \cdot \vec{v}_2 - \frac{21}{64} \hat{n} \times \vec{S}_1 \cdot \vec{v}_1 \vec{v}_2 \cdot \vec{v}_2 + \frac{27}{128} \hat{n} \times \vec{S}_1 \cdot \vec{v}_2 \vec{v}_2 \cdot \vec{v}_2 \right) \left. \right) m_1 m_2^2 G^3 \}
\end{aligned}$$

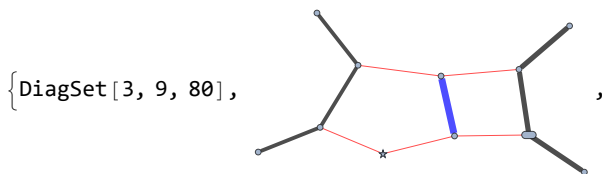

$$\begin{aligned}
& \frac{G^3 m_1 m_2^2 \left( 3 \hat{n} \cdot \vec{v}_2 \hat{n} \times \vec{S}_1 \cdot \vec{a}_1 - \frac{7}{3} \vec{S}_1 \times \vec{a}_1 \cdot \vec{v}_2 + 3 \hat{n} \cdot \vec{v}_2 \hat{n} \times \vec{S}_1 \cdot \vec{v}_1 - \frac{7}{3} \vec{S}_1 \times \vec{v}_1 \cdot \vec{v}_2 \right)}{r^3} + \frac{1}{r^4} \\
& G^3 m_1 m_2^2 \left( 21 (\hat{n} \cdot \vec{v}_2)^2 \hat{n} \times \vec{S}_1 \cdot \vec{v}_1 - 10 \hat{n} \cdot \vec{v}_2 \vec{S}_1 \times \vec{v}_1 \cdot \vec{v}_2 - 15 \hat{n} \cdot \vec{v}_1 \hat{n} \cdot \vec{v}_2 \hat{n} \times \vec{S}_1 \cdot \vec{v}_1 + 7 \hat{n} \cdot \vec{v}_1 \vec{S}_1 \times \vec{v}_1 \cdot \vec{v}_2 + \right. \\
& \quad \left. 3 \vec{v}_1 \cdot \vec{v}_2 \hat{n} \times \vec{S}_1 \cdot \vec{v}_1 - \vec{v}_2 \cdot \vec{v}_2 \hat{n} \times \vec{S}_1 \cdot \vec{v}_1 + \pi^2 \left( -\frac{15}{8} (\hat{n} \cdot \vec{v}_2)^2 \hat{n} \times \vec{S}_1 \cdot \vec{v}_1 + \frac{3}{4} \hat{n} \cdot \vec{v}_2 \vec{S}_1 \times \vec{v}_1 \cdot \vec{v}_2 + \frac{3}{8} \vec{v}_2 \cdot \vec{v}_2 \hat{n} \times \vec{S}_1 \cdot \vec{v}_1 \right) \right) \}
\end{aligned}$$

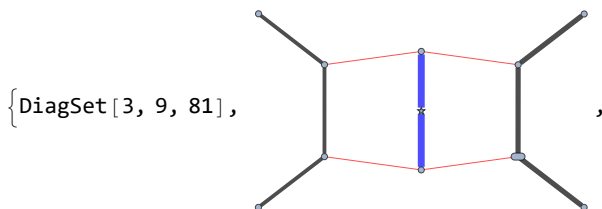

$$\begin{aligned}
& \frac{1}{r^3} G^3 m_1 m_2^2 \left( \frac{14}{3} \hat{n} \cdot \vec{v}_1 \hat{n} \times \vec{a}_1 \cdot \vec{S}_1 - \frac{35}{3} \hat{n} \cdot \vec{v}_2 \hat{n} \times \vec{a}_1 \cdot \vec{S}_1 + \pi^2 \left( \frac{3}{4} \hat{n} \cdot \vec{v}_2 \hat{n} \times \vec{a}_1 \cdot \vec{S}_1 - \frac{1}{4} \vec{a}_1 \times \vec{S}_1 \cdot \vec{v}_2 - \frac{3}{4} \hat{n} \cdot \vec{v}_2 \hat{n} \times \vec{S}_1 \cdot \vec{v}_1 + \right. \right. \\
& \quad \left. \left. \frac{1}{4} \vec{S}_1 \times \vec{v}_1 \cdot \vec{v}_2 \right) - \frac{14}{9} \vec{a}_1 \times \vec{S}_1 \cdot \vec{v}_1 + \frac{47}{9} \vec{a}_1 \times \vec{S}_1 \cdot \vec{v}_2 - \frac{14}{3} \hat{n} \cdot \vec{v}_1 \hat{n} \times \vec{S}_1 \cdot \vec{v}_1 + \frac{35}{3} \hat{n} \cdot \vec{v}_2 \hat{n} \times \vec{S}_1 \cdot \vec{v}_1 - \frac{47}{9} \vec{S}_1 \times \vec{v}_1 \cdot \vec{v}_2 \right) + \\
& \frac{1}{r^4} G^3 m_1 m_2^2 \left( \frac{35}{3} (\hat{n} \cdot \vec{v}_1)^2 \hat{n} \times \vec{S}_1 \cdot \vec{v}_1 + \frac{35}{3} \hat{n} \cdot \vec{v}_1 \vec{S}_1 \times \vec{v}_1 \cdot \vec{v}_2 - \frac{175}{3} \hat{n} \cdot \vec{v}_2 \hat{n} \cdot \vec{v}_1 \hat{n} \times \vec{S}_1 \cdot \vec{v}_1 + \right. \\
& \quad \frac{35}{3} (\hat{n} \cdot \vec{v}_2)^2 \hat{n} \times \vec{S}_1 \cdot \vec{v}_1 - \frac{14}{3} \hat{n} \cdot \vec{v}_2 \vec{S}_1 \times \vec{v}_1 \cdot \vec{v}_2 - \frac{7}{3} \vec{v}_1 \cdot \vec{v}_1 \hat{n} \times \vec{S}_1 \cdot \vec{v}_1 + \frac{47}{3} \vec{v}_1 \cdot \vec{v}_2 \hat{n} \times \vec{S}_1 \cdot \vec{v}_1 + \\
& \quad \left. \pi^2 \left( -\frac{3}{4} \hat{n} \cdot \vec{v}_1 \vec{S}_1 \times \vec{v}_1 \cdot \vec{v}_2 + \frac{15}{4} \hat{n} \cdot \vec{v}_2 \hat{n} \cdot \vec{v}_1 \hat{n} \times \vec{S}_1 \cdot \vec{v}_1 - \frac{3}{4} \vec{v}_1 \cdot \vec{v}_2 \hat{n} \times \vec{S}_1 \cdot \vec{v}_1 \right) - \frac{7}{3} \vec{v}_2 \cdot \vec{v}_2 \hat{n} \times \vec{S}_1 \cdot \vec{v}_1 \right) \}
\end{aligned}$$



{DiagSet[3, 9, 82],

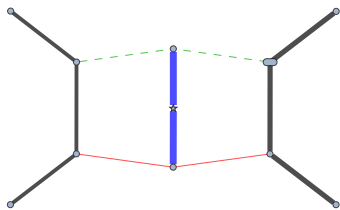

,

$$\begin{aligned} & \frac{1}{r^3} \left( -\frac{13}{9} \vec{S}_1 \times \vec{v}_1 \cdot \vec{v}_2 - \frac{13}{9} \vec{S}_1 \times \vec{v}_1 \cdot \vec{a}_2 + \frac{7}{9} \vec{S}_1 \times \vec{v}_2 \cdot \vec{a}_2 - \frac{10}{3} \hat{n} \times \vec{S}_1 \cdot \vec{v}_1 \hat{n} \cdot \vec{a}_2 + \right. \\ & \quad \frac{10}{3} \hat{n} \times \vec{S}_1 \cdot \vec{v}_2 \hat{n} \cdot \vec{a}_2 - \frac{23}{3} \hat{n} \times \vec{S}_1 \cdot \vec{v}_2 \hat{n} \cdot \vec{v}_1 - \frac{23}{3} \hat{n} \times \vec{S}_1 \cdot \vec{a}_2 \hat{n} \cdot \vec{v}_1 - \frac{10}{3} \hat{n} \times \vec{S}_1 \cdot \vec{v}_1 \hat{n} \cdot \vec{v}_2 + \\ & \quad 13 \hat{n} \times \vec{S}_1 \cdot \vec{v}_2 \hat{n} \cdot \vec{v}_2 + \frac{29}{3} \hat{n} \times \vec{S}_1 \cdot \vec{a}_2 \hat{n} \cdot \vec{v}_2 + \pi^2 \left( \frac{1}{4} \vec{S}_1 \times \vec{v}_1 \cdot \vec{v}_2 + \frac{1}{4} \vec{S}_1 \times \vec{v}_1 \cdot \vec{a}_2 - \frac{1}{4} \vec{S}_1 \times \vec{v}_2 \cdot \vec{a}_2 + \right. \\ & \quad \left. \frac{3}{4} \hat{n} \times \vec{S}_1 \cdot \vec{v}_2 \hat{n} \cdot \vec{v}_1 + \frac{3}{4} \hat{n} \times \vec{S}_1 \cdot \vec{a}_2 \hat{n} \cdot \vec{v}_1 - \frac{3}{4} \hat{n} \times \vec{S}_1 \cdot \vec{v}_2 \hat{n} \cdot \vec{v}_2 - \frac{3}{4} \hat{n} \times \vec{S}_1 \cdot \vec{a}_2 \hat{n} \cdot \vec{v}_2 \right) \Big) m_1 m_2^2 G^3 + \frac{1}{r^4} \\ & \left( \frac{83}{6} \hat{n} \times \vec{S}_1 \cdot \vec{v}_2 (\hat{n} \cdot \vec{v}_1)^2 + \frac{26}{3} \vec{S}_1 \times \vec{v}_1 \cdot \vec{v}_2 \hat{n} \cdot \vec{v}_1 - \frac{47}{3} \hat{n} \times \vec{S}_1 \cdot \vec{v}_1 \hat{n} \cdot \vec{v}_2 \hat{n} \cdot \vec{v}_1 + \frac{238}{3} \hat{n} \times \vec{S}_1 \cdot \vec{v}_2 \hat{n} \cdot \vec{v}_2 \hat{n} \cdot \vec{v}_1 - \right. \\ & \quad \frac{116}{3} \hat{n} \times \vec{S}_1 \cdot \vec{v}_1 (\hat{n} \cdot \vec{v}_2)^2 + \frac{73}{6} \hat{n} \times \vec{S}_1 \cdot \vec{v}_2 (\hat{n} \cdot \vec{v}_2)^2 + \frac{82}{3} \vec{S}_1 \times \vec{v}_1 \cdot \vec{v}_2 \hat{n} \cdot \vec{v}_2 - \frac{7}{6} \hat{n} \times \vec{S}_1 \cdot \vec{v}_2 \vec{v}_1 \cdot \vec{v}_1 + \\ & \quad \frac{19}{3} \hat{n} \times \vec{S}_1 \cdot \vec{v}_1 \vec{v}_1 \cdot \vec{v}_2 - \frac{98}{3} \hat{n} \times \vec{S}_1 \cdot \vec{v}_2 \vec{v}_1 \cdot \vec{v}_2 + \frac{28}{3} \hat{n} \times \vec{S}_1 \cdot \vec{v}_1 \vec{v}_2 \cdot \vec{v}_2 + \frac{19}{6} \hat{n} \times \vec{S}_1 \cdot \vec{v}_2 \vec{v}_2 \cdot \vec{v}_2 + \\ & \quad \pi^2 \left( -\frac{45}{32} \hat{n} \times \vec{S}_1 \cdot \vec{v}_2 (\hat{n} \cdot \vec{v}_1)^2 - \frac{3}{4} \vec{S}_1 \times \vec{v}_1 \cdot \vec{v}_2 \hat{n} \cdot \vec{v}_1 + \frac{15}{16} \hat{n} \times \vec{S}_1 \cdot \vec{v}_1 \hat{n} \cdot \vec{v}_2 \hat{n} \cdot \vec{v}_1 - \frac{15}{2} \hat{n} \times \vec{S}_1 \cdot \vec{v}_2 \hat{n} \cdot \vec{v}_2 \hat{n} \cdot \vec{v}_1 + \right. \\ & \quad \frac{15}{4} \hat{n} \times \vec{S}_1 \cdot \vec{v}_1 (\hat{n} \cdot \vec{v}_2)^2 - \frac{45}{32} \hat{n} \times \vec{S}_1 \cdot \vec{v}_2 (\hat{n} \cdot \vec{v}_2)^2 - 3 \vec{S}_1 \times \vec{v}_1 \cdot \vec{v}_2 \hat{n} \cdot \vec{v}_2 + \frac{9}{32} \hat{n} \times \vec{S}_1 \cdot \vec{v}_2 \vec{v}_1 \cdot \vec{v}_1 - \\ & \quad \left. \frac{3}{16} \hat{n} \times \vec{S}_1 \cdot \vec{v}_1 \vec{v}_1 \cdot \vec{v}_2 + \frac{3}{2} \hat{n} \times \vec{S}_1 \cdot \vec{v}_2 \vec{v}_1 \cdot \vec{v}_2 - \frac{3}{4} \hat{n} \times \vec{S}_1 \cdot \vec{v}_1 \vec{v}_2 \cdot \vec{v}_2 + \frac{9}{32} \hat{n} \times \vec{S}_1 \cdot \vec{v}_2 \vec{v}_2 \cdot \vec{v}_2 \right) \Big) m_1 m_2^2 G^3 \Big\} \end{aligned}$$

{DiagSet[3, 9, 83],

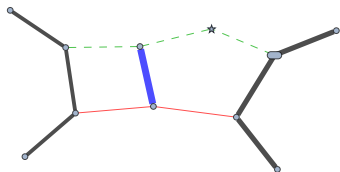

,

$$\begin{aligned} & \left( \frac{\frac{1}{4} \pi^2 \hat{n} \times \vec{S}_1 \cdot \vec{a}_2 - 3 \hat{n} \times \vec{S}_1 \cdot \vec{a}_2}{r^2} + \frac{1}{r^3} \left( -\frac{14}{3} \vec{S}_1 \times \vec{v}_1 \cdot \vec{v}_2 + \frac{23}{3} \vec{S}_1 \times \vec{v}_1 \cdot \vec{a}_2 - \right. \right. \\ & \quad 11 \hat{n} \times \vec{S}_1 \cdot \vec{v}_1 \hat{n} \cdot \vec{a}_2 + 5 \hat{n} \times \vec{S}_1 \cdot \vec{v}_2 \hat{n} \cdot \vec{v}_1 + 4 \hat{n} \times \vec{S}_1 \cdot \vec{a}_2 \hat{n} \cdot \vec{v}_1 + 11 \hat{n} \times \vec{S}_1 \cdot \vec{v}_1 \hat{n} \cdot \vec{v}_2 - 9 \hat{n} \times \vec{S}_1 \cdot \vec{v}_2 \hat{n} \cdot \vec{v}_2 + \\ & \quad \left. \pi^2 \left( -\frac{1}{4} \vec{S}_1 \times \vec{v}_1 \cdot \vec{a}_2 + \frac{3}{4} \hat{n} \times \vec{S}_1 \cdot \vec{v}_1 \hat{n} \cdot \vec{a}_2 - \frac{3}{4} \hat{n} \times \vec{S}_1 \cdot \vec{v}_2 \hat{n} \cdot \vec{v}_1 - \frac{3}{4} \hat{n} \times \vec{S}_1 \cdot \vec{v}_1 \hat{n} \cdot \vec{v}_2 + \frac{3}{4} \hat{n} \times \vec{S}_1 \cdot \vec{v}_2 \hat{n} \cdot \vec{v}_2 \right) \right) m_1 m_2^2 G^3 + \\ & \frac{1}{r^4} \left( -\frac{107}{12} \hat{n} \times \vec{S}_1 \cdot \vec{v}_2 (\hat{n} \cdot \vec{v}_1)^2 - \frac{35}{3} \vec{S}_1 \times \vec{v}_1 \cdot \vec{v}_2 \hat{n} \cdot \vec{v}_1 + \frac{49}{2} \hat{n} \times \vec{S}_1 \cdot \vec{v}_1 \hat{n} \cdot \vec{v}_2 \hat{n} \cdot \vec{v}_1 + 20 \hat{n} \times \vec{S}_1 \cdot \vec{v}_2 \hat{n} \cdot \vec{v}_2 \hat{n} \cdot \vec{v}_1 - \right. \\ & \quad 55 \hat{n} \times \vec{S}_1 \cdot \vec{v}_1 (\hat{n} \cdot \vec{v}_2)^2 + 34 \vec{S}_1 \times \vec{v}_1 \cdot \vec{v}_2 \hat{n} \cdot \vec{v}_2 - \frac{17}{12} \hat{n} \times \vec{S}_1 \cdot \vec{v}_2 \vec{v}_1 \cdot \vec{v}_1 - \frac{13}{2} \hat{n} \times \vec{S}_1 \cdot \vec{v}_1 \vec{v}_1 \cdot \vec{v}_2 - 4 \hat{n} \times \vec{S}_1 \cdot \vec{v}_2 \vec{v}_1 \cdot \vec{v}_2 + \\ & \quad 11 \hat{n} \times \vec{S}_1 \cdot \vec{v}_1 \vec{v}_2 \cdot \vec{v}_2 + \pi^2 \left( \frac{45}{64} \hat{n} \times \vec{S}_1 \cdot \vec{v}_2 (\hat{n} \cdot \vec{v}_1)^2 + \frac{3}{4} \vec{S}_1 \times \vec{v}_1 \cdot \vec{v}_2 \hat{n} \cdot \vec{v}_1 - \frac{75}{32} \hat{n} \times \vec{S}_1 \cdot \vec{v}_1 \hat{n} \cdot \vec{v}_2 \hat{n} \cdot \vec{v}_1 + \frac{15}{4} \hat{n} \times \vec{S}_1 \cdot \vec{v}_1 \right. \\ & \quad \left. (\hat{n} \cdot \vec{v}_2)^2 - \frac{3}{2} \vec{S}_1 \times \vec{v}_1 \cdot \vec{v}_2 \hat{n} \cdot \vec{v}_2 - \frac{9}{64} \hat{n} \times \vec{S}_1 \cdot \vec{v}_2 \vec{v}_1 \cdot \vec{v}_1 + \frac{15}{32} \hat{n} \times \vec{S}_1 \cdot \vec{v}_1 \vec{v}_1 \cdot \vec{v}_2 - \frac{3}{4} \hat{n} \times \vec{S}_1 \cdot \vec{v}_1 \vec{v}_2 \cdot \vec{v}_2 \right) \Big) m_1 m_2^2 G^3 \Big\} \end{aligned}$$

{DiagSet[3, 9, 84],

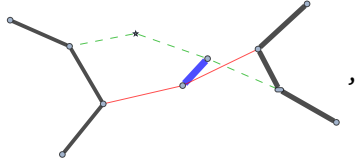

,

$$\begin{aligned} & \frac{1}{r^3} G^3 m_1 m_2^2 \left( -14 \hat{n} \cdot \vec{a}_2 \hat{n} \times \vec{S}_1 \cdot \vec{v}_2 + 22 \hat{n} \cdot \vec{v}_1 \hat{n} \times \vec{S}_1 \cdot \vec{a}_2 - 12 \hat{n} \cdot \vec{v}_2 \hat{n} \times \vec{S}_1 \cdot \vec{a}_2 + \pi^2 \right. \\ & \left( \frac{3}{4} \hat{n} \cdot \vec{a}_2 \hat{n} \times \vec{S}_1 \cdot \vec{v}_2 - \frac{3}{2} \hat{n} \cdot \vec{v}_1 \hat{n} \times \vec{S}_1 \cdot \vec{a}_2 + \frac{3}{2} \hat{n} \cdot \vec{v}_2 \hat{n} \times \vec{S}_1 \cdot \vec{a}_2 - \frac{1}{2} \vec{S}_1 \times \vec{v}_1 \cdot \vec{a}_2 + \frac{1}{4} \vec{S}_1 \times \vec{v}_2 \cdot \vec{a}_2 - \frac{3}{4} \hat{n} \cdot \vec{v}_2 \hat{n} \times \vec{S}_1 \cdot \vec{v}_2 \right) + \\ & \frac{22}{3} \vec{S}_1 \times \vec{v}_1 \cdot \vec{a}_2 + 2 \vec{S}_1 \times \vec{v}_2 \cdot \vec{a}_2 + 4 \hat{n} \cdot \vec{v}_2 \hat{n} \times \vec{S}_1 \cdot \vec{v}_2 \left. \right) + \frac{G^3 m_1 m_2^2 \left( \frac{1}{2} \pi^2 \hat{n} \times \vec{S}_1 \cdot \vec{a}_2 - \frac{22}{3} \hat{n} \times \vec{S}_1 \cdot \vec{a}_2 \right)}{r^2} + \frac{1}{r^4} \\ & G^3 m_1 m_2^2 \left( (\hat{n} \cdot \vec{v}_2)^2 \left( -(\hat{n} \times \vec{S}_1 \cdot \vec{v}_2) \right) - 4 \hat{n} \cdot \vec{v}_2 \vec{S}_1 \times \vec{v}_1 \cdot \vec{v}_2 - 20 \hat{n} \cdot \vec{v}_1 \hat{n} \cdot \vec{v}_2 \hat{n} \times \vec{S}_1 \cdot \vec{v}_2 + 4 \vec{v}_1 \cdot \vec{v}_2 \hat{n} \times \vec{S}_1 \cdot \vec{v}_2 + \right. \\ & \left. \pi^2 \left( \frac{3}{4} \hat{n} \cdot \vec{v}_2 \vec{S}_1 \times \vec{v}_1 \cdot \vec{v}_2 + \frac{15}{4} \hat{n} \cdot \vec{v}_1 \hat{n} \cdot \vec{v}_2 \hat{n} \times \vec{S}_1 \cdot \vec{v}_2 - \frac{3}{4} \vec{v}_1 \cdot \vec{v}_2 \hat{n} \times \vec{S}_1 \cdot \vec{v}_2 \right) - 7 \vec{v}_2 \cdot \vec{v}_2 \hat{n} \times \vec{S}_1 \cdot \vec{v}_2 \right) \} \end{aligned}$$

{DiagSet[3, 9, 85],

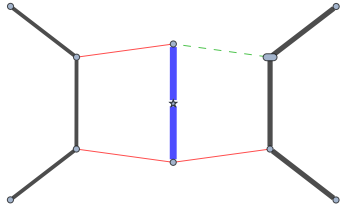

,

$$\begin{aligned} & \left( -\frac{8}{9} \hat{n} \times \vec{S}_1 \cdot \vec{v}_1 - \frac{1}{4} \pi^2 \hat{n} \times \vec{S}_1 \cdot \vec{v}_2 + \frac{35}{9} \hat{n} \times \vec{S}_1 \cdot \vec{v}_2 \right) m_1 m_2^2 G^3 \\ & \frac{1}{r^3} \left( 12 \vec{S}_1 \times \vec{v}_1 \cdot \vec{v}_2 - \frac{8}{9} \vec{a}_1 \times \vec{S}_1 \cdot \vec{v}_1 - \frac{11}{18} \vec{a}_1 \times \vec{S}_1 \cdot \vec{v}_2 + \frac{97}{18} \vec{a}_2 \times \vec{S}_1 \cdot \vec{v}_1 - \frac{35}{9} \vec{a}_2 \times \vec{S}_1 \cdot \vec{v}_2 + \frac{4}{3} \hat{n} \times \vec{S}_1 \cdot \vec{v}_1 \hat{n} \cdot \vec{a}_1 - \right. \\ & \frac{4}{3} \hat{n} \times \vec{S}_1 \cdot \vec{v}_2 \hat{n} \cdot \vec{a}_1 - \frac{9}{2} \hat{n} \times \vec{S}_1 \cdot \vec{v}_1 \hat{n} \cdot \vec{a}_2 + \frac{31}{6} \hat{n} \times \vec{S}_1 \cdot \vec{v}_2 \hat{n} \cdot \vec{a}_2 + \frac{52}{3} \hat{n} \times \vec{S}_1 \cdot \vec{v}_2 \hat{n} \cdot \vec{v}_1 + \frac{4}{3} \hat{n} \times \vec{a}_1 \cdot \vec{S}_1 \hat{n} \cdot \vec{v}_1 - \\ & \frac{29}{3} \hat{n} \times \vec{a}_2 \cdot \vec{S}_1 \hat{n} \cdot \vec{v}_1 - \frac{50}{3} \hat{n} \times \vec{S}_1 \cdot \vec{v}_1 \hat{n} \cdot \vec{v}_2 - \frac{4}{3} \hat{n} \times \vec{S}_1 \cdot \vec{v}_2 \hat{n} \cdot \vec{v}_2 + \frac{19}{6} \hat{n} \times \vec{a}_1 \cdot \vec{S}_1 \hat{n} \cdot \vec{v}_2 + \frac{13}{2} \hat{n} \times \vec{a}_2 \cdot \vec{S}_1 \hat{n} \cdot \vec{v}_2 + \\ & \pi^2 \left( -\left( \frac{1}{\vec{S}_1 \times \vec{v}_1 \cdot \vec{v}_2} \right) + \frac{1}{8} \vec{a}_1 \times \vec{S}_1 \cdot \vec{v}_2 - \frac{3}{8} \vec{a}_2 \times \vec{S}_1 \cdot \vec{v}_1 + \frac{1}{4} \vec{a}_2 \times \vec{S}_1 \cdot \vec{v}_2 + \frac{3}{8} \hat{n} \times \vec{S}_1 \cdot \vec{v}_1 \hat{n} \cdot \vec{a}_2 - \frac{3}{8} \hat{n} \times \vec{S}_1 \cdot \vec{v}_2 \hat{n} \cdot \vec{a}_2 - \right. \\ & \left. \frac{3}{2} \hat{n} \times \vec{S}_1 \cdot \vec{v}_2 \hat{n} \cdot \vec{v}_1 + \frac{3}{4} \hat{n} \times \vec{a}_2 \cdot \vec{S}_1 \hat{n} \cdot \vec{v}_1 + \frac{3}{2} \hat{n} \times \vec{S}_1 \cdot \vec{v}_1 \hat{n} \cdot \vec{v}_2 - \frac{3}{8} \hat{n} \times \vec{a}_1 \cdot \vec{S}_1 \hat{n} \cdot \vec{v}_2 - \frac{3}{8} \hat{n} \times \vec{a}_2 \cdot \vec{S}_1 \hat{n} \cdot \vec{v}_2 \right) \left. \right) m_1 m_2^2 G^3 + \\ & \frac{1}{r^4} \left( -\frac{20}{3} \hat{n} \times \vec{S}_1 \cdot \vec{v}_1 (\hat{n} \cdot \vec{v}_1)^2 - \frac{373}{12} \hat{n} \times \vec{S}_1 \cdot \vec{v}_2 (\hat{n} \cdot \vec{v}_1)^2 - \frac{89}{3} \vec{S}_1 \times \vec{v}_1 \cdot \vec{v}_2 \hat{n} \cdot \vec{v}_1 + \frac{469}{6} \hat{n} \times \vec{S}_1 \cdot \vec{v}_1 \hat{n} \cdot \vec{v}_2 \hat{n} \cdot \vec{v}_1 - \right. \\ & \frac{269}{3} \hat{n} \times \vec{S}_1 \cdot \vec{v}_2 \hat{n} \cdot \vec{v}_2 \hat{n} \cdot \vec{v}_1 + \frac{101}{3} \hat{n} \times \vec{S}_1 \cdot \vec{v}_1 (\hat{n} \cdot \vec{v}_2)^2 + \frac{49}{12} \hat{n} \times \vec{S}_1 \cdot \vec{v}_2 (\hat{n} \cdot \vec{v}_2)^2 - \\ & 29 \vec{S}_1 \times \vec{v}_1 \cdot \vec{v}_2 \hat{n} \cdot \vec{v}_2 + \frac{4}{3} \hat{n} \times \vec{S}_1 \cdot \vec{v}_1 \vec{v}_1 \cdot \vec{v}_1 + \frac{41}{12} \hat{n} \times \vec{S}_1 \cdot \vec{v}_2 \vec{v}_1 \cdot \vec{v}_1 - \frac{149}{6} \hat{n} \times \vec{S}_1 \cdot \vec{v}_1 \vec{v}_1 \cdot \vec{v}_2 + \\ & \frac{97}{3} \hat{n} \times \vec{S}_1 \cdot \vec{v}_2 \vec{v}_1 \cdot \vec{v}_2 - \frac{19}{3} \hat{n} \times \vec{S}_1 \cdot \vec{v}_1 \vec{v}_2 \cdot \vec{v}_2 - \frac{53}{12} \hat{n} \times \vec{S}_1 \cdot \vec{v}_2 \vec{v}_2 \cdot \vec{v}_2 + \\ & \pi^2 \left( \frac{225}{64} \hat{n} \times \vec{S}_1 \cdot \vec{v}_2 (\hat{n} \cdot \vec{v}_1)^2 + \frac{21}{8} \vec{S}_1 \times \vec{v}_1 \cdot \vec{v}_2 \hat{n} \cdot \vec{v}_1 - \frac{195}{32} \hat{n} \times \vec{S}_1 \cdot \vec{v}_1 \hat{n} \cdot \vec{v}_2 \hat{n} \cdot \vec{v}_1 + \frac{15}{2} \hat{n} \times \vec{S}_1 \cdot \vec{v}_2 \hat{n} \cdot \vec{v}_2 \hat{n} \cdot \vec{v}_1 - \right. \\ & \frac{15}{4} \hat{n} \times \vec{S}_1 \cdot \vec{v}_1 (\hat{n} \cdot \vec{v}_2)^2 + \frac{15}{64} \hat{n} \times \vec{S}_1 \cdot \vec{v}_2 (\hat{n} \cdot \vec{v}_2)^2 + 3 \vec{S}_1 \times \vec{v}_1 \cdot \vec{v}_2 \hat{n} \cdot \vec{v}_2 - \frac{45}{64} \hat{n} \times \vec{S}_1 \cdot \vec{v}_2 \vec{v}_1 \cdot \vec{v}_1 + \\ & \left. \frac{39}{32} \hat{n} \times \vec{S}_1 \cdot \vec{v}_1 \vec{v}_1 \cdot \vec{v}_2 - \frac{3}{2} \hat{n} \times \vec{S}_1 \cdot \vec{v}_2 \vec{v}_1 \cdot \vec{v}_2 + \frac{3}{4} \hat{n} \times \vec{S}_1 \cdot \vec{v}_1 \vec{v}_2 \cdot \vec{v}_2 - \frac{3}{64} \hat{n} \times \vec{S}_1 \cdot \vec{v}_2 \vec{v}_2 \cdot \vec{v}_2 \right) \left. \right) m_1 m_2^2 G^3 \} \end{aligned}$$

{DiagSet[3, 9, 86],

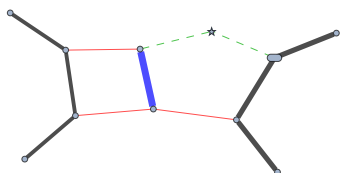

,

$$\frac{\left(5 \hat{n} \times \vec{S}_1 \cdot \vec{v}_1 + \pi^2 \left( \frac{1}{8} \hat{n} \times \vec{a}_2 \cdot \vec{S}_1 - \frac{1}{4} \hat{n} \times \vec{S}_1 \cdot \vec{v}_1 \right) - \frac{5}{2} \hat{n} \times \vec{a}_2 \cdot \vec{S}_1 \right) m_1 m_2^2 G^3}{r^2} + \frac{1}{r^3}$$

$$\left( 3 \vec{S}_1 \times \vec{v}_1 \cdot \vec{v}_2 + 5 \vec{a}_1 \times \vec{S}_1 \cdot \vec{v}_1 - 5 \vec{a}_1 \times \vec{S}_1 \cdot \vec{v}_2 + \frac{9}{2} \vec{a}_2 \times \vec{S}_1 \cdot \vec{v}_1 - \frac{5}{3} \hat{n} \times \vec{S}_1 \cdot \vec{v}_1 \hat{n} \cdot \vec{a}_1 - \frac{55}{6} \hat{n} \times \vec{S}_1 \cdot \vec{v}_1 \hat{n} \cdot \vec{a}_2 + \right.$$

$$\frac{70}{3} \hat{n} \times \vec{S}_1 \cdot \vec{v}_1 \hat{n} \cdot \vec{v}_1 - \frac{83}{6} \hat{n} \times \vec{S}_1 \cdot \vec{v}_2 \hat{n} \cdot \vec{v}_1 - \frac{40}{3} \hat{n} \times \vec{a}_1 \cdot \vec{S}_1 \hat{n} \cdot \vec{v}_1 - \frac{19}{3} \hat{n} \times \vec{a}_2 \cdot \vec{S}_1 \hat{n} \cdot \vec{v}_1 - \frac{125}{6} \hat{n} \times \vec{S}_1 \cdot \vec{v}_1 \hat{n} \cdot \vec{v}_2 +$$

$$\frac{15}{2} \hat{n} \times \vec{S}_1 \cdot \vec{v}_2 \hat{n} \cdot \vec{v}_2 + 15 \hat{n} \times \vec{a}_1 \cdot \vec{S}_1 \hat{n} \cdot \vec{v}_2 + \pi^2 \left( \frac{1}{8} \vec{S}_1 \times \vec{v}_1 \cdot \vec{v}_2 - \frac{1}{4} \vec{a}_1 \times \vec{S}_1 \cdot \vec{v}_1 + \frac{1}{4} \vec{a}_1 \times \vec{S}_1 \cdot \vec{v}_2 - \right.$$

$$\frac{1}{2} \vec{a}_2 \times \vec{S}_1 \cdot \vec{v}_1 + \frac{3}{4} \hat{n} \times \vec{S}_1 \cdot \vec{v}_1 \hat{n} \cdot \vec{a}_2 - \frac{3}{2} \hat{n} \times \vec{S}_1 \cdot \vec{v}_1 \hat{n} \cdot \vec{v}_1 + \frac{9}{8} \hat{n} \times \vec{S}_1 \cdot \vec{v}_2 \hat{n} \cdot \vec{v}_1 + \frac{3}{4} \hat{n} \times \vec{a}_1 \cdot \vec{S}_1 \hat{n} \cdot \vec{v}_1 +$$

$$\left. \frac{3}{4} \hat{n} \times \vec{a}_2 \cdot \vec{S}_1 \hat{n} \cdot \vec{v}_1 + \frac{3}{4} \hat{n} \times \vec{S}_1 \cdot \vec{v}_1 \hat{n} \cdot \vec{v}_2 - \frac{3}{8} \hat{n} \times \vec{S}_1 \cdot \vec{v}_2 \hat{n} \cdot \vec{v}_2 - \frac{3}{4} \hat{n} \times \vec{a}_1 \cdot \vec{S}_1 \hat{n} \cdot \vec{v}_2 \right) m_1 m_2^2 G^3 + \frac{1}{r^4}$$

$$\left( -\frac{107}{12} \hat{n} \times \vec{S}_1 \cdot \vec{v}_1 (\hat{n} \cdot \vec{v}_1)^2 - \frac{75}{8} \hat{n} \times \vec{S}_1 \cdot \vec{v}_2 (\hat{n} \cdot \vec{v}_1)^2 - \frac{49}{6} \vec{S}_1 \times \vec{v}_1 \cdot \vec{v}_2 \hat{n} \cdot \vec{v}_1 + \frac{313}{12} \hat{n} \times \vec{S}_1 \cdot \vec{v}_1 \hat{n} \cdot \vec{v}_2 \hat{n} \cdot \vec{v}_1 + \right.$$

$$\frac{95}{3} \hat{n} \times \vec{S}_1 \cdot \vec{v}_2 \hat{n} \cdot \vec{v}_2 \hat{n} \cdot \vec{v}_1 - \frac{275}{6} \hat{n} \times \vec{S}_1 \cdot \vec{v}_1 (\hat{n} \cdot \vec{v}_2)^2 + \frac{68}{3} \vec{S}_1 \times \vec{v}_1 \cdot \vec{v}_2 \hat{n} \cdot \vec{v}_2 - \frac{65}{12} \hat{n} \times \vec{S}_1 \cdot \vec{v}_1 \vec{v}_1 \cdot \vec{v}_1 +$$

$$\frac{31}{8} \hat{n} \times \vec{S}_1 \cdot \vec{v}_2 \vec{v}_1 \cdot \vec{v}_1 - \frac{29}{12} \hat{n} \times \vec{S}_1 \cdot \vec{v}_1 \vec{v}_1 \cdot \vec{v}_2 - \frac{19}{3} \hat{n} \times \vec{S}_1 \cdot \vec{v}_2 \vec{v}_1 \cdot \vec{v}_2 + \frac{55}{6} \hat{n} \times \vec{S}_1 \cdot \vec{v}_1 \vec{v}_2 \cdot \vec{v}_2 +$$

$$\pi^2 \left( \frac{45}{64} \hat{n} \times \vec{S}_1 \cdot \vec{v}_1 (\hat{n} \cdot \vec{v}_1)^2 + \frac{135}{128} \hat{n} \times \vec{S}_1 \cdot \vec{v}_2 (\hat{n} \cdot \vec{v}_1)^2 + \frac{9}{16} \vec{S}_1 \times \vec{v}_1 \cdot \vec{v}_2 \hat{n} \cdot \vec{v}_1 - \frac{45}{64} \hat{n} \times \vec{S}_1 \cdot \vec{v}_1 \hat{n} \cdot \vec{v}_2 \hat{n} \cdot \vec{v}_1 - \right.$$

$$\frac{15}{4} \hat{n} \times \vec{S}_1 \cdot \vec{v}_2 \hat{n} \cdot \vec{v}_2 \hat{n} \cdot \vec{v}_1 + \frac{15}{4} \hat{n} \times \vec{S}_1 \cdot \vec{v}_1 (\hat{n} \cdot \vec{v}_2)^2 - \frac{9}{4} \vec{S}_1 \times \vec{v}_1 \cdot \vec{v}_2 \hat{n} \cdot \vec{v}_2 - \frac{9}{64} \hat{n} \times \vec{S}_1 \cdot \vec{v}_1 \vec{v}_1 \cdot \vec{v}_1 -$$

$$\left. \frac{27}{128} \hat{n} \times \vec{S}_1 \cdot \vec{v}_2 \vec{v}_1 \cdot \vec{v}_1 + \frac{9}{64} \hat{n} \times \vec{S}_1 \cdot \vec{v}_1 \vec{v}_1 \cdot \vec{v}_2 + \frac{3}{4} \hat{n} \times \vec{S}_1 \cdot \vec{v}_2 \vec{v}_1 \cdot \vec{v}_2 - \frac{3}{4} \hat{n} \times \vec{S}_1 \cdot \vec{v}_1 \vec{v}_2 \cdot \vec{v}_2 \right) m_1 m_2^2 G^3 \}$$

{DiagSet[3, 9, 87],

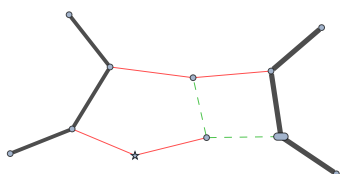

,

$$\frac{1}{r^3} \left( \frac{1}{2} \vec{S}_1 \times \vec{v}_1 \cdot \vec{v}_2 + \frac{1}{2} \vec{S}_1 \times \vec{a}_1 \cdot \vec{v}_2 + \frac{1}{2} \vec{S}_1 \times \vec{v}_2 \cdot \vec{a}_2 + \frac{1}{2} \hat{n} \times \vec{S}_1 \cdot \vec{v}_2 \hat{n} \cdot \vec{a}_1 - 2 \hat{n} \times \vec{S}_1 \cdot \vec{v}_2 \hat{n} \cdot \vec{a}_2 + \frac{1}{2} \hat{n} \times \vec{S}_1 \cdot \vec{v}_2 \hat{n} \cdot \vec{v}_1 - \right.$$

$$\frac{5}{2} \hat{n} \times \vec{S}_1 \cdot \vec{v}_2 \hat{n} \cdot \vec{v}_2 - \frac{1}{2} \hat{n} \times \vec{S}_1 \cdot \vec{a}_2 \hat{n} \cdot \vec{v}_2 + \pi^2 \left( -\frac{1}{16} \vec{S}_1 \times \vec{v}_1 \cdot \vec{v}_2 - \frac{1}{16} \vec{S}_1 \times \vec{a}_1 \cdot \vec{v}_2 - \frac{1}{8} \vec{S}_1 \times \vec{v}_2 \cdot \vec{a}_2 + \right.$$

$$\left. \frac{3}{8} \hat{n} \times \vec{S}_1 \cdot \vec{v}_2 \hat{n} \cdot \vec{a}_2 + \frac{3}{16} \hat{n} \times \vec{S}_1 \cdot \vec{v}_1 \hat{n} \cdot \vec{v}_2 + \frac{3}{8} \hat{n} \times \vec{S}_1 \cdot \vec{v}_2 \hat{n} \cdot \vec{v}_2 + \frac{3}{16} \hat{n} \times \vec{S}_1 \cdot \vec{a}_1 \hat{n} \cdot \vec{v}_2 \right) m_1 m_2^2 G^3 +$$

$$\frac{1}{r^4} \left( -\frac{5}{2} \hat{n} \times \vec{S}_1 \cdot \vec{v}_2 (\hat{n} \cdot \vec{v}_1)^2 - 2 \vec{S}_1 \times \vec{v}_1 \cdot \vec{v}_2 \hat{n} \cdot \vec{v}_1 + \frac{21}{2} \hat{n} \times \vec{S}_1 \cdot \vec{v}_2 \hat{n} \cdot \vec{v}_2 \hat{n} \cdot \vec{v}_1 - \frac{5}{4} \hat{n} \times \vec{S}_1 \cdot \vec{v}_1 (\hat{n} \cdot \vec{v}_2)^2 - \right.$$

$$\frac{83}{8} \hat{n} \times \vec{S}_1 \cdot \vec{v}_2 (\hat{n} \cdot \vec{v}_2)^2 + 3 \vec{S}_1 \times \vec{v}_1 \cdot \vec{v}_2 \hat{n} \cdot \vec{v}_2 + \frac{1}{2} \hat{n} \times \vec{S}_1 \cdot \vec{v}_2 \vec{v}_1 \cdot \vec{v}_1 - \frac{5}{2} \hat{n} \times \vec{S}_1 \cdot \vec{v}_2 \vec{v}_1 \cdot \vec{v}_2 +$$

$$\frac{5}{4} \hat{n} \times \vec{S}_1 \cdot \vec{v}_1 \vec{v}_2 \cdot \vec{v}_2 + \frac{7}{8} \hat{n} \times \vec{S}_1 \cdot \vec{v}_2 \vec{v}_2 \cdot \vec{v}_2 + \pi^2 \left( \frac{45}{64} \hat{n} \times \vec{S}_1 \cdot \vec{v}_1 (\hat{n} \cdot \vec{v}_2)^2 + \frac{195}{128} \hat{n} \times \vec{S}_1 \cdot \vec{v}_2 (\hat{n} \cdot \vec{v}_2)^2 - \right.$$

$$\left. \frac{9}{16} \vec{S}_1 \times \vec{v}_1 \cdot \vec{v}_2 \hat{n} \cdot \vec{v}_2 - \frac{15}{16} \hat{n} \times \vec{S}_1 \cdot \vec{v}_1 \hat{n} \cdot \vec{v}_1 \hat{n} \cdot \vec{v}_2 - \frac{45}{32} \hat{n} \times \vec{S}_1 \cdot \vec{v}_2 \hat{n} \cdot \vec{v}_1 \hat{n} \cdot \vec{v}_2 + \frac{3}{16} \vec{S}_1 \times \vec{v}_1 \cdot \vec{v}_2 \hat{n} \cdot \vec{v}_1 + \right.$$

$$\left. \left. \frac{3}{16} \hat{n} \times \vec{S}_1 \cdot \vec{v}_1 \vec{v}_1 \cdot \vec{v}_2 + \frac{9}{32} \hat{n} \times \vec{S}_1 \cdot \vec{v}_2 \vec{v}_1 \cdot \vec{v}_2 - \frac{9}{64} \hat{n} \times \vec{S}_1 \cdot \vec{v}_1 \vec{v}_2 \cdot \vec{v}_2 - \frac{39}{128} \hat{n} \times \vec{S}_1 \cdot \vec{v}_2 \vec{v}_2 \cdot \vec{v}_2 \right) \right\} m_1 m_2^2 G^3 \}$$

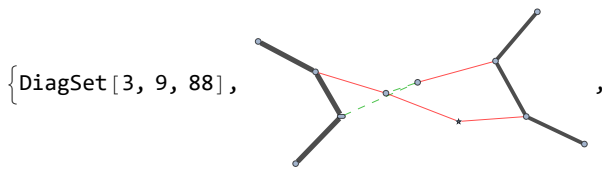

$$\frac{\left( \frac{1}{2} \hat{n} \times \vec{S}_1 \cdot \vec{a}_2 - \frac{1}{8} \pi^2 \hat{n} \times \vec{S}_1 \cdot \vec{a}_2 \right) m_1 m_2^2 G^3}{r^2} + \frac{1}{r^3} \left( - \left( \frac{1}{\vec{S}_1 \times \vec{v}_1 \cdot \vec{v}_2} \right) - \vec{S}_1 \times \vec{a}_1 \cdot \vec{v}_2 - \frac{1}{2} \vec{S}_1 \times \vec{v}_1 \cdot \vec{a}_2 + \frac{1}{2} \vec{S}_1 \times \vec{v}_2 \cdot \vec{a}_2 + \right. \\ \left. \frac{1}{2} \hat{n} \times \vec{S}_1 \cdot \vec{v}_2 \hat{n} \cdot \vec{a}_1 + \frac{1}{2} \hat{n} \times \vec{S}_1 \cdot \vec{v}_2 \hat{n} \cdot \vec{a}_2 + \frac{1}{2} \hat{n} \times \vec{S}_1 \cdot \vec{v}_2 \hat{n} \cdot \vec{v}_1 - \frac{3}{2} \hat{n} \times \vec{S}_1 \cdot \vec{a}_2 \hat{n} \cdot \vec{v}_1 + \frac{5}{2} \hat{n} \times \vec{S}_1 \cdot \vec{v}_1 \hat{n} \cdot \vec{v}_2 - \right. \\ \left. \hat{n} \times \vec{S}_1 \cdot \vec{v}_2 \hat{n} \cdot \vec{v}_2 + \frac{5}{2} \hat{n} \times \vec{S}_1 \cdot \vec{a}_1 \hat{n} \cdot \vec{v}_2 + 2 \hat{n} \times \vec{S}_1 \cdot \vec{a}_2 \hat{n} \cdot \vec{v}_2 + \pi^2 \left( \frac{1}{16} \vec{S}_1 \times \vec{v}_1 \cdot \vec{v}_2 + \frac{1}{16} \vec{S}_1 \times \vec{a}_1 \cdot \vec{v}_2 + \frac{1}{8} \vec{S}_1 \times \vec{v}_1 \cdot \vec{a}_2 - \right. \right. \\ \left. \left. \frac{1}{8} \vec{S}_1 \times \vec{v}_2 \cdot \vec{a}_2 + \frac{3}{8} \hat{n} \times \vec{S}_1 \cdot \vec{a}_2 \hat{n} \cdot \vec{v}_1 - \frac{3}{16} \hat{n} \times \vec{S}_1 \cdot \vec{v}_1 \hat{n} \cdot \vec{v}_2 - \frac{3}{16} \hat{n} \times \vec{S}_1 \cdot \vec{a}_1 \hat{n} \cdot \vec{v}_2 - \frac{3}{8} \hat{n} \times \vec{S}_1 \cdot \vec{a}_2 \hat{n} \cdot \vec{v}_2 \right) \right) m_1 m_2^2 G^3 + \\ \frac{1}{r^4} \left( - \frac{5}{2} \hat{n} \times \vec{S}_1 \cdot \vec{v}_2 (\hat{n} \cdot \vec{v}_1)^2 + \frac{5}{2} \vec{S}_1 \times \vec{v}_1 \cdot \vec{v}_2 \hat{n} \cdot \vec{v}_1 - \frac{25}{2} \hat{n} \times \vec{S}_1 \cdot \vec{v}_1 \hat{n} \cdot \vec{v}_2 \hat{n} \cdot \vec{v}_1 + 3 \hat{n} \times \vec{S}_1 \cdot \vec{v}_2 \hat{n} \cdot \vec{v}_2 \hat{n} \cdot \vec{v}_1 + \right. \\ \left. \frac{37}{4} \hat{n} \times \vec{S}_1 \cdot \vec{v}_1 (\hat{n} \cdot \vec{v}_2)^2 + \frac{17}{8} \hat{n} \times \vec{S}_1 \cdot \vec{v}_2 (\hat{n} \cdot \vec{v}_2)^2 - \frac{7}{2} \vec{S}_1 \times \vec{v}_1 \cdot \vec{v}_2 \hat{n} \cdot \vec{v}_2 + \frac{1}{2} \hat{n} \times \vec{S}_1 \cdot \vec{v}_2 \vec{v}_1 \cdot \vec{v}_1 + \right. \\ \left. \frac{5}{2} \hat{n} \times \vec{S}_1 \cdot \vec{v}_1 \vec{v}_1 \cdot \vec{v}_2 - \hat{n} \times \vec{S}_1 \cdot \vec{v}_2 \vec{v}_1 \cdot \vec{v}_2 - \frac{5}{4} \hat{n} \times \vec{S}_1 \cdot \vec{v}_1 \vec{v}_2 \cdot \vec{v}_2 - \frac{13}{8} \hat{n} \times \vec{S}_1 \cdot \vec{v}_2 \vec{v}_2 \cdot \vec{v}_2 + \right. \\ \left. \pi^2 \left( - \frac{75}{64} \hat{n} \times \vec{S}_1 \cdot \vec{v}_1 (\hat{n} \cdot \vec{v}_2)^2 - \frac{45}{128} \hat{n} \times \vec{S}_1 \cdot \vec{v}_2 (\hat{n} \cdot \vec{v}_2)^2 + \frac{9}{16} \vec{S}_1 \times \vec{v}_1 \cdot \vec{v}_2 \hat{n} \cdot \vec{v}_2 + \right. \right. \\ \left. \left. \frac{15}{16} \hat{n} \times \vec{S}_1 \cdot \vec{v}_1 \hat{n} \cdot \vec{v}_1 \hat{n} \cdot \vec{v}_2 + \frac{15}{32} \hat{n} \times \vec{S}_1 \cdot \vec{v}_2 \hat{n} \cdot \vec{v}_1 \hat{n} \cdot \vec{v}_2 - \frac{3}{16} \vec{S}_1 \times \vec{v}_1 \cdot \vec{v}_2 \hat{n} \cdot \vec{v}_1 - \frac{3}{16} \hat{n} \times \vec{S}_1 \cdot \vec{v}_1 \vec{v}_1 \cdot \vec{v}_2 - \right. \right. \\ \left. \left. \frac{3}{32} \hat{n} \times \vec{S}_1 \cdot \vec{v}_2 \vec{v}_1 \cdot \vec{v}_2 + \frac{15}{64} \hat{n} \times \vec{S}_1 \cdot \vec{v}_1 \vec{v}_2 \cdot \vec{v}_2 + \frac{9}{128} \hat{n} \times \vec{S}_1 \cdot \vec{v}_2 \vec{v}_2 \cdot \vec{v}_2 \right) \right) m_1 m_2^2 G^3 \}$$

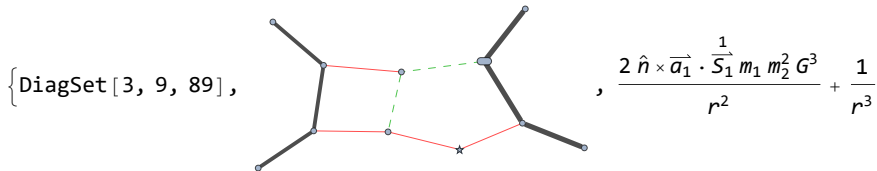

$$\frac{2 \hat{n} \times \vec{a}_1 \cdot \vec{S}_1 m_1 m_2^2 G^3}{r^2} + \frac{1}{r^3} \\ \left( - \frac{1}{2} \vec{S}_1 \times \vec{v}_1 \cdot \vec{v}_2 + 2 \vec{a}_1 \times \vec{S}_1 \cdot \vec{v}_1 - 2 \vec{a}_1 \times \vec{S}_1 \cdot \vec{v}_2 - \frac{1}{2} \vec{a}_2 \times \vec{S}_1 \cdot \vec{v}_1 - \hat{n} \times \vec{S}_1 \cdot \vec{v}_1 \hat{n} \cdot \vec{a}_1 + 2 \hat{n} \times \vec{S}_1 \cdot \vec{v}_1 \hat{n} \cdot \vec{a}_2 + 2 \hat{n} \times \vec{S}_1 \cdot \vec{v}_1 \hat{n} \cdot \vec{v}_1 + \right. \\ \left. \frac{5}{2} \hat{n} \times \vec{S}_1 \cdot \vec{v}_2 \hat{n} \cdot \vec{v}_1 - 5 \hat{n} \times \vec{a}_1 \cdot \vec{S}_1 \hat{n} \cdot \vec{v}_1 - \frac{5}{2} \hat{n} \times \vec{a}_2 \cdot \vec{S}_1 \hat{n} \cdot \vec{v}_1 + 2 \hat{n} \times \vec{S}_1 \cdot \vec{v}_1 \hat{n} \cdot \vec{v}_2 + 6 \hat{n} \times \vec{a}_1 \cdot \vec{S}_1 \hat{n} \cdot \vec{v}_2 + \pi^2 \right. \\ \left. \left( - \frac{1}{4} \vec{S}_1 \times \vec{v}_1 \cdot \vec{v}_2 - \frac{1}{4} \vec{a}_2 \times \vec{S}_1 \cdot \vec{v}_1 + \frac{3}{8} \hat{n} \times \vec{S}_1 \cdot \vec{v}_1 \hat{n} \cdot \vec{a}_2 - \frac{3}{8} \hat{n} \times \vec{S}_1 \cdot \vec{v}_2 \hat{n} \cdot \vec{v}_1 + \frac{3}{8} \hat{n} \times \vec{a}_2 \cdot \vec{S}_1 \hat{n} \cdot \vec{v}_1 + \frac{3}{8} \hat{n} \times \vec{S}_1 \cdot \vec{v}_1 \hat{n} \cdot \vec{v}_2 \right) \right) \\ m_1 m_2^2 G^3 + \frac{1}{r^4} \left( - 4 \hat{n} \times \vec{S}_1 \cdot \vec{v}_1 (\hat{n} \cdot \vec{v}_1)^2 - \frac{83}{8} \hat{n} \times \vec{S}_1 \cdot \vec{v}_2 (\hat{n} \cdot \vec{v}_1)^2 - 5 \vec{S}_1 \times \vec{v}_1 \cdot \vec{v}_2 \hat{n} \cdot \vec{v}_1 + \frac{33}{4} \hat{n} \times \vec{S}_1 \cdot \vec{v}_1 \hat{n} \cdot \vec{v}_2 \hat{n} \cdot \vec{v}_1 + \right. \\ \left. \frac{25}{2} \hat{n} \times \vec{S}_1 \cdot \vec{v}_2 \hat{n} \cdot \vec{v}_2 \hat{n} \cdot \vec{v}_1 + 10 \hat{n} \times \vec{S}_1 \cdot \vec{v}_1 (\hat{n} \cdot \vec{v}_2)^2 - \frac{7}{2} \vec{S}_1 \times \vec{v}_1 \cdot \vec{v}_2 \hat{n} \cdot \vec{v}_2 + 2 \hat{n} \times \vec{S}_1 \cdot \vec{v}_1 \vec{v}_1 \cdot \vec{v}_1 + \frac{7}{8} \hat{n} \times \vec{S}_1 \cdot \vec{v}_2 \vec{v}_1 \cdot \vec{v}_1 - \right. \\ \left. \frac{5}{4} \hat{n} \times \vec{S}_1 \cdot \vec{v}_1 \vec{v}_1 \cdot \vec{v}_2 - \frac{5}{2} \hat{n} \times \vec{S}_1 \cdot \vec{v}_2 \vec{v}_1 \cdot \vec{v}_2 - 2 \hat{n} \times \vec{S}_1 \cdot \vec{v}_1 \vec{v}_2 \cdot \vec{v}_2 + \pi^2 \left( \frac{195}{128} \hat{n} \times \vec{S}_1 \cdot \vec{v}_2 (\hat{n} \cdot \vec{v}_1)^2 + \frac{15}{16} \vec{S}_1 \times \vec{v}_1 \cdot \vec{v}_2 \hat{n} \cdot \vec{v}_1 - \right. \right. \\ \left. \left. \frac{105}{64} \hat{n} \times \vec{S}_1 \cdot \vec{v}_1 \hat{n} \cdot \vec{v}_2 \hat{n} \cdot \vec{v}_1 - \frac{15}{8} \hat{n} \times \vec{S}_1 \cdot \vec{v}_2 \hat{n} \cdot \vec{v}_2 \hat{n} \cdot \vec{v}_1 + \frac{15}{8} \hat{n} \times \vec{S}_1 \cdot \vec{v}_1 (\hat{n} \cdot \vec{v}_2)^2 - \frac{9}{8} \vec{S}_1 \times \vec{v}_1 \cdot \vec{v}_2 \hat{n} \cdot \vec{v}_2 - \right. \right. \\ \left. \left. \frac{39}{128} \hat{n} \times \vec{S}_1 \cdot \vec{v}_2 \vec{v}_1 \cdot \vec{v}_1 + \frac{21}{64} \hat{n} \times \vec{S}_1 \cdot \vec{v}_1 \vec{v}_1 \cdot \vec{v}_2 + \frac{3}{8} \hat{n} \times \vec{S}_1 \cdot \vec{v}_2 \vec{v}_1 \cdot \vec{v}_2 - \frac{3}{8} \hat{n} \times \vec{S}_1 \cdot \vec{v}_1 \vec{v}_2 \cdot \vec{v}_2 \right) \right) m_1 m_2^2 G^3 \}$$

{DiagSet[3, 9, 90],

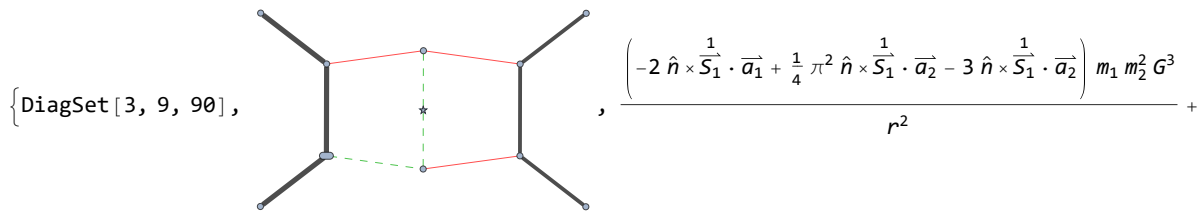

, 
$$\frac{\left(-2 \hat{n} \times \vec{S}_1 \cdot \vec{a}_1 + \frac{1}{4} \pi^2 \hat{n} \times \vec{S}_1 \cdot \vec{a}_2 - 3 \hat{n} \times \vec{S}_1 \cdot \vec{a}_2\right) m_1 m_2^2 G^3}{r^2} +$$

$$\begin{aligned} & \frac{1}{r^3} \left( -\frac{3}{2} \vec{S}_1 \times \vec{a}_1 \cdot \vec{v}_2 + 2 \vec{S}_1 \times \vec{v}_1 \cdot \vec{a}_1 + \frac{13}{2} \vec{S}_1 \times \vec{v}_1 \cdot \vec{a}_2 - 3 \vec{S}_1 \times \vec{v}_2 \cdot \vec{a}_2 - 3 \hat{n} \times \vec{S}_1 \cdot \vec{v}_1 \hat{n} \cdot \vec{a}_1 - \frac{17}{2} \hat{n} \times \vec{S}_1 \cdot \vec{v}_1 \hat{n} \cdot \vec{a}_2 + \right. \\ & \quad \frac{9}{2} \hat{n} \times \vec{S}_1 \cdot \vec{v}_2 \hat{n} \cdot \vec{a}_2 + 6 \hat{n} \times \vec{S}_1 \cdot \vec{v}_1 \hat{n} \cdot \vec{v}_1 + 3 \hat{n} \times \vec{S}_1 \cdot \vec{a}_1 \hat{n} \cdot \vec{v}_1 + 9 \hat{n} \times \vec{S}_1 \cdot \vec{a}_2 \hat{n} \cdot \vec{v}_1 - 9 \hat{n} \times \vec{S}_1 \cdot \vec{v}_2 \hat{n} \cdot \vec{v}_2 + \\ & \quad \frac{5}{2} \hat{n} \times \vec{S}_1 \cdot \vec{a}_1 \hat{n} \cdot \vec{v}_2 - \frac{9}{2} \hat{n} \times \vec{S}_1 \cdot \vec{a}_2 \hat{n} \cdot \vec{v}_2 + \pi^2 \left( \frac{1}{8} \vec{S}_1 \times \vec{a}_1 \cdot \vec{v}_2 - \frac{3}{8} \vec{S}_1 \times \vec{v}_1 \cdot \vec{a}_2 + \frac{1}{4} \vec{S}_1 \times \vec{v}_2 \cdot \vec{a}_2 + \frac{3}{8} \hat{n} \times \vec{S}_1 \cdot \vec{v}_1 \hat{n} \cdot \vec{a}_2 - \right. \\ & \quad \left. \frac{3}{8} \hat{n} \times \vec{S}_1 \cdot \vec{v}_2 \hat{n} \cdot \vec{a}_2 - \frac{3}{4} \hat{n} \times \vec{S}_1 \cdot \vec{a}_2 \hat{n} \cdot \vec{v}_1 + \frac{3}{4} \hat{n} \times \vec{S}_1 \cdot \vec{v}_2 \hat{n} \cdot \vec{v}_2 - \frac{3}{8} \hat{n} \times \vec{S}_1 \cdot \vec{a}_1 \hat{n} \cdot \vec{v}_2 + \frac{3}{8} \hat{n} \times \vec{S}_1 \cdot \vec{a}_2 \hat{n} \cdot \vec{v}_2 \right) \Big) m_1 m_2^2 G^3 + \\ & \frac{1}{r^4} \left( \frac{9}{4} \hat{n} \times \vec{S}_1 \cdot \vec{v}_2 (\hat{n} \cdot \vec{v}_1)^2 + 5 \vec{S}_1 \times \vec{v}_1 \cdot \vec{v}_2 \hat{n} \cdot \vec{v}_1 - \frac{21}{2} \hat{n} \times \vec{S}_1 \cdot \vec{v}_1 \hat{n} \cdot \vec{v}_2 \hat{n} \cdot \vec{v}_1 + 24 \hat{n} \times \vec{S}_1 \cdot \vec{v}_2 \hat{n} \cdot \vec{v}_2 \hat{n} \cdot \vec{v}_1 - \right. \\ & \quad 28 \hat{n} \times \vec{S}_1 \cdot \vec{v}_1 (\hat{n} \cdot \vec{v}_2)^2 - \frac{9}{4} \hat{n} \times \vec{S}_1 \cdot \vec{v}_2 (\hat{n} \cdot \vec{v}_2)^2 + 18 \vec{S}_1 \times \vec{v}_1 \cdot \vec{v}_2 \hat{n} \cdot \vec{v}_2 + \frac{3}{4} \hat{n} \times \vec{S}_1 \cdot \vec{v}_2 \vec{v}_1 \cdot \vec{v}_1 + \\ & \quad \frac{5}{2} \hat{n} \times \vec{S}_1 \cdot \vec{v}_1 \vec{v}_1 \cdot \vec{v}_2 - 4 \hat{n} \times \vec{S}_1 \cdot \vec{v}_2 \vec{v}_1 \cdot \vec{v}_2 + 6 \hat{n} \times \vec{S}_1 \cdot \vec{v}_1 \vec{v}_2 \cdot \vec{v}_2 - \frac{3}{4} \hat{n} \times \vec{S}_1 \cdot \vec{v}_2 \vec{v}_2 \cdot \vec{v}_2 + \\ & \quad \pi^2 \left( -\frac{15}{64} \hat{n} \times \vec{S}_1 \cdot \vec{v}_2 (\hat{n} \cdot \vec{v}_1)^2 - \frac{3}{8} \vec{S}_1 \times \vec{v}_1 \cdot \vec{v}_2 \hat{n} \cdot \vec{v}_1 + \frac{45}{32} \hat{n} \times \vec{S}_1 \cdot \vec{v}_1 \hat{n} \cdot \vec{v}_2 \hat{n} \cdot \vec{v}_1 - \frac{15}{8} \hat{n} \times \vec{S}_1 \cdot \vec{v}_2 \hat{n} \cdot \vec{v}_2 \hat{n} \cdot \vec{v}_1 + \right. \\ & \quad \frac{15}{16} \hat{n} \times \vec{S}_1 \cdot \vec{v}_1 (\hat{n} \cdot \vec{v}_2)^2 + \frac{15}{64} \hat{n} \times \vec{S}_1 \cdot \vec{v}_2 (\hat{n} \cdot \vec{v}_2)^2 - \frac{3}{4} \vec{S}_1 \times \vec{v}_1 \cdot \vec{v}_2 \hat{n} \cdot \vec{v}_2 + \frac{3}{64} \hat{n} \times \vec{S}_1 \cdot \vec{v}_2 \vec{v}_1 \cdot \vec{v}_1 - \\ & \quad \left. \frac{9}{32} \hat{n} \times \vec{S}_1 \cdot \vec{v}_1 \vec{v}_1 \cdot \vec{v}_2 + \frac{3}{8} \hat{n} \times \vec{S}_1 \cdot \vec{v}_2 \vec{v}_1 \cdot \vec{v}_2 - \frac{3}{16} \hat{n} \times \vec{S}_1 \cdot \vec{v}_1 \vec{v}_2 \cdot \vec{v}_2 - \frac{3}{64} \hat{n} \times \vec{S}_1 \cdot \vec{v}_2 \vec{v}_2 \cdot \vec{v}_2 \right) \Big) m_1 m_2^2 G^3 \Big\} \end{aligned}$$

{DiagSet[3, 9, 91],

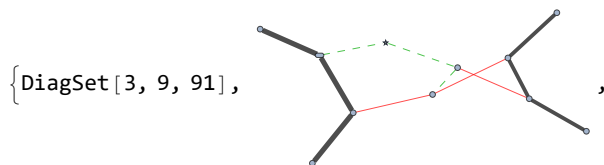

,

$$\begin{aligned} & \frac{\left( \hat{n} \times \vec{S}_1 \cdot \vec{a}_1 + \pi^2 \left( \frac{1}{8} \hat{n} \times \vec{S}_1 \cdot \vec{a}_2 - \frac{1}{4} \hat{n} \times \vec{S}_1 \cdot \vec{a}_1 \right) - \frac{1}{2} \hat{n} \times \vec{S}_1 \cdot \vec{a}_2 \right) m_1 m_2^2 G^3}{r^2} + \frac{1}{r^3} \\ & \left( -\left( \vec{S}_1 \times \vec{v}_1 \cdot \vec{a}_1 \right) - \frac{1}{2} \vec{S}_1 \times \vec{v}_1 \cdot \vec{a}_2 + \hat{n} \times \vec{S}_1 \cdot \vec{v}_1 \hat{n} \cdot \vec{a}_1 + \frac{7}{2} \hat{n} \times \vec{S}_1 \cdot \vec{v}_1 \hat{n} \cdot \vec{a}_2 - 2 \hat{n} \times \vec{S}_1 \cdot \vec{v}_1 \hat{n} \cdot \vec{v}_1 + \right. \\ & \quad \frac{3}{2} \hat{n} \times \vec{S}_1 \cdot \vec{v}_2 \hat{n} \cdot \vec{v}_1 - 2 \hat{n} \times \vec{S}_1 \cdot \vec{a}_1 \hat{n} \cdot \vec{v}_1 - \frac{1}{2} \hat{n} \times \vec{S}_1 \cdot \vec{v}_1 \hat{n} \cdot \vec{v}_2 - \frac{3}{2} \hat{n} \times \vec{S}_1 \cdot \vec{v}_2 \hat{n} \cdot \vec{v}_2 + \\ & \quad \pi^2 \left( -\frac{1}{8} \vec{S}_1 \times \vec{v}_1 \cdot \vec{v}_2 + \frac{1}{4} \vec{S}_1 \times \vec{v}_1 \cdot \vec{a}_1 + \frac{1}{4} \vec{S}_1 \times \vec{v}_1 \cdot \vec{a}_2 - \frac{3}{8} \hat{n} \times \vec{S}_1 \cdot \vec{v}_1 \hat{n} \cdot \vec{a}_1 - \frac{3}{4} \hat{n} \times \vec{S}_1 \cdot \vec{v}_1 \hat{n} \cdot \vec{a}_2 + \right. \\ & \quad \left. \frac{3}{4} \hat{n} \times \vec{S}_1 \cdot \vec{v}_1 \hat{n} \cdot \vec{v}_1 - \frac{3}{8} \hat{n} \times \vec{S}_1 \cdot \vec{v}_2 \hat{n} \cdot \vec{v}_1 + \frac{3}{8} \hat{n} \times \vec{S}_1 \cdot \vec{a}_1 \hat{n} \cdot \vec{v}_1 + \frac{3}{8} \hat{n} \times \vec{S}_1 \cdot \vec{v}_2 \hat{n} \cdot \vec{v}_2 \right) \Big) m_1 m_2^2 G^3 + \\ & \frac{1}{r^4} \left( \frac{19}{4} \hat{n} \times \vec{S}_1 \cdot \vec{v}_1 (\hat{n} \cdot \vec{v}_1)^2 + \frac{19}{8} \hat{n} \times \vec{S}_1 \cdot \vec{v}_2 (\hat{n} \cdot \vec{v}_1)^2 + \frac{3}{2} \vec{S}_1 \times \vec{v}_1 \cdot \vec{v}_2 \hat{n} \cdot \vec{v}_1 - \frac{27}{4} \hat{n} \times \vec{S}_1 \cdot \vec{v}_1 \hat{n} \cdot \vec{v}_2 \hat{n} \cdot \vec{v}_1 + \right. \\ & \quad \frac{35}{2} \hat{n} \times \vec{S}_1 \cdot \vec{v}_1 (\hat{n} \cdot \vec{v}_2)^2 - 5 \vec{S}_1 \times \vec{v}_1 \cdot \vec{v}_2 \hat{n} \cdot \vec{v}_2 + \frac{1}{4} \hat{n} \times \vec{S}_1 \cdot \vec{v}_1 \vec{v}_1 \cdot \vec{v}_1 - \frac{7}{8} \hat{n} \times \vec{S}_1 \cdot \vec{v}_2 \vec{v}_1 \cdot \vec{v}_1 + \\ & \quad \frac{7}{4} \hat{n} \times \vec{S}_1 \cdot \vec{v}_1 \vec{v}_1 \cdot \vec{v}_2 - \frac{7}{2} \hat{n} \times \vec{S}_1 \cdot \vec{v}_1 \vec{v}_2 \cdot \vec{v}_2 + \pi^2 \left( -\frac{15}{64} \hat{n} \times \vec{S}_1 \cdot \vec{v}_1 (\hat{n} \cdot \vec{v}_1)^2 - \frac{15}{128} \hat{n} \times \vec{S}_1 \cdot \vec{v}_2 (\hat{n} \cdot \vec{v}_1)^2 - \right. \\ & \quad \left. \frac{3}{16} \vec{S}_1 \times \vec{v}_1 \cdot \vec{v}_2 \hat{n} \cdot \vec{v}_1 + \frac{45}{64} \hat{n} \times \vec{S}_1 \cdot \vec{v}_1 \hat{n} \cdot \vec{v}_2 \hat{n} \cdot \vec{v}_1 - \frac{15}{4} \hat{n} \times \vec{S}_1 \cdot \vec{v}_1 (\hat{n} \cdot \vec{v}_2)^2 + \frac{3}{2} \vec{S}_1 \times \vec{v}_1 \cdot \vec{v}_2 \hat{n} \cdot \vec{v}_2 + \right. \end{aligned}$$

$$\frac{3}{64} \hat{n} \times \vec{S}_1 \cdot \vec{v}_1 \vec{v}_1 \cdot \vec{v}_1 + \frac{3}{128} \hat{n} \times \vec{S}_1 \cdot \vec{v}_2 \vec{v}_1 \cdot \vec{v}_1 - \frac{9}{64} \hat{n} \times \vec{S}_1 \cdot \vec{v}_1 \vec{v}_1 \cdot \vec{v}_2 + \frac{3}{4} \hat{n} \times \vec{S}_1 \cdot \vec{v}_1 \vec{v}_2 \cdot \vec{v}_2 \Bigg) \Bigg) m_1 m_2^2 G^3 \Bigg\}$$
